# Supplementary material for: N$^3$LO Quadratic-in-Spin Interactions for Generic Compact Binaries
Source: arXiv:2209.09235 ancillary file (2023-01-27)
Supplement: Supplementary file 1 [file frules-wl-vis.pdf]

Worldline vertex rules.

Worldline time integration has been suppressed.

Spin variable presented in spin-tensor form.

Legends :

- 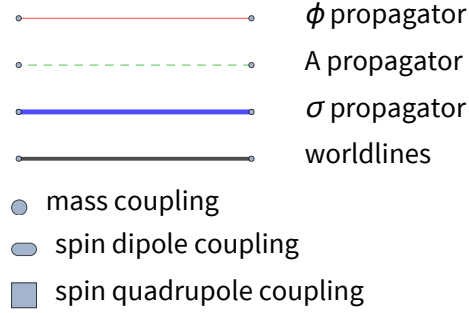  $\phi$  propagator
- 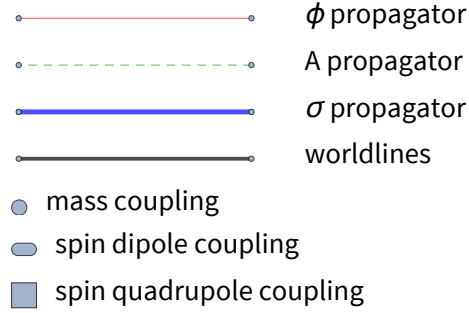 A propagator
- 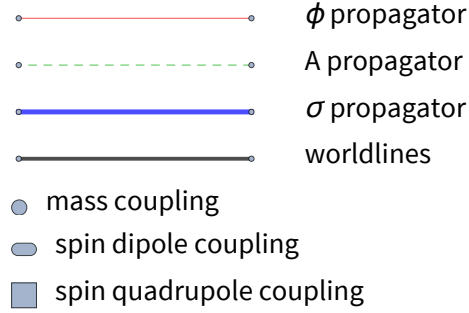  $\sigma$  propagator
- 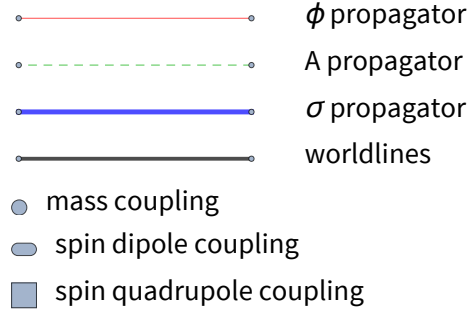 worldlines
- 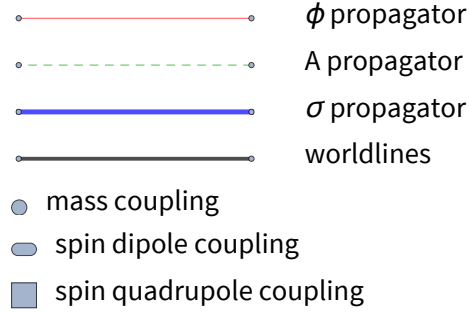 mass coupling
- 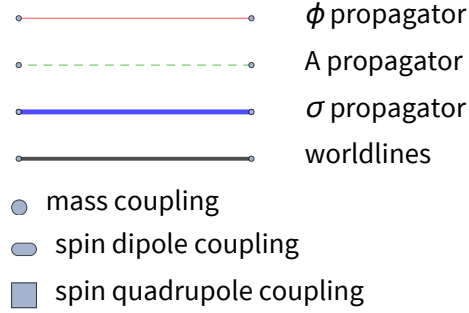 spin dipole coupling
- 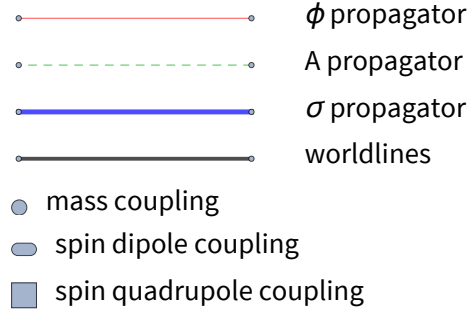 spin quadrupole coupling

$$\left\{ \text{Kinetic term, } -\frac{m}{(c^{-1})^2} + \frac{1}{2} m (v_i v^i) + \frac{1}{8} (c^{-1})^2 m (v_i v^i)^2 + \right. \\ \left. \frac{1}{16} (c^{-1})^4 m (v_i v^i)^3 + \frac{5}{128} (c^{-1})^6 m (v_i v^i)^4 + \frac{7}{256} (c^{-1})^8 m (v_i v^i)^5 \right\} \\ \left\{ \text{Kinetic term, } -\frac{1}{2} (c^{-1})^3 (a^i S_{ii1} v^{i1}) - \frac{3}{8} (c^{-1})^5 (v_i v^i) (a^i S_{ii1} v^{i1}) - \right. \\ \left. \frac{5}{16} (c^{-1})^7 (v_i v^i)^2 (a^i S_{ii1} v^{i1}) - \frac{35}{128} (c^{-1})^9 (v_i v^i)^3 (a^i S_{ii1} v^{i1}) \right\}$$

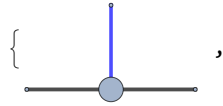

$$\frac{1}{2} (c^{-1})^4 m (v^i v^{i1} \sigma_{ii1}) + \frac{1}{4} (c^{-1})^6 m (v_i v^i) (v^i v^{i1} \sigma_{ii1}) + \frac{3}{16} (c^{-1})^8 m (v_i v^i)^2 (v^i v^{i1} \sigma_{ii1}) \Big\}$$

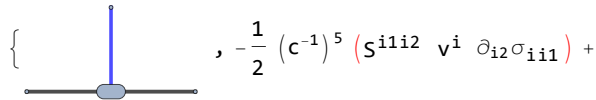

$$\frac{1}{4} (c^{-1})^7 \left( (a^i S_{ii1}^{i2} v^{i1} \sigma_{ii2}) - (a^i S_i^{i2} v^{i1} \sigma_{ii2}) + 2 (S_i^{i3} v^i v^{i1} v^{i2} \partial_{i2} \sigma_{ii3}) - \right. \\ \left. (S_i^{i3} v^i v^{i1} v^{i2} \partial_{i3} \sigma_{ii2}) + 3 (S_i^{i2} v^i v^{i1} \partial_t \sigma_{ii2}) \right) + \\ \frac{1}{16} (c^{-1})^9 \left( -6 (a^i S_{ii1} v^{i1}) (v^i v^{i1} \sigma_{ii1}) + (v_i v^i) (3 (a^i S_{ii1}^{i2} v^{i1} \sigma_{ii2}) - 3 (a^i S_i^{i2} v^{i1} \sigma_{ii2}) + \right. \\ \left. 6 (S_i^{i3} v^i v^{i1} v^{i2} \partial_{i2} \sigma_{ii3}) - 3 (S_i^{i3} v^i v^{i1} v^{i2} \partial_{i3} \sigma_{ii2}) + 7 (S_i^{i2} v^i v^{i1} \partial_t \sigma_{ii2}) \right) \Big\}$$

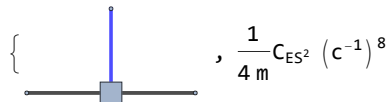

$$\left( 2 (S_{ii1}^{i3} S_{ii2}^{i2} v^i \partial_i \partial_t \sigma_{ii2}) + (S_{ii2}^{i4} S_{ii3}^{i2} v^i v^{i1} \partial_{ii1} \partial_i \sigma_{ii3}) - 2 (S_{ii1}^{i3} S_{ii2}^{i2} v^i \partial_{i3} \partial_t \sigma_{ii2}) - \right. \\ \left. 2 (S_{ii2}^{i4} S_{ii3}^{i2} v^i v^{i1} \partial_{i4} \partial_{ii1} \sigma_{ii3}) + (S_{ii2}^{i4} S_{ii3}^{i2} v^i v^{i1} \partial_{i4} \partial_{i3} \sigma_{ii1}) + (S_i^{i2} S_{ii1}^{i3} \partial_t \partial_t \sigma_{ii2}) \right) +$$

$$\frac{1}{8m} C_{ES^2} (c^{-1})^{10} \left( (v_i v^i) \left( 2 (S_{i1}^{i3} S^{i1i2} v^i \partial_i \partial_t \sigma_{i2i3}) + (S_{i2}^{i4} S^{i2i3} v^i v^{i1} \partial_{i1} \partial_i \sigma_{i3i4}) - \right. \right. \\ \left. \left. 2 (S_{i1}^{i3} S^{i1i2} v^i \partial_{i3} \partial_t \sigma_{i1i2}) - 2 (S_{i2}^{i4} S^{i2i3} v^i v^{i1} \partial_{i4} \partial_{i1} \sigma_{i1i3}) + \right. \right. \\ \left. \left. (S_{i2}^{i4} S^{i2i3} v^i v^{i1} \partial_{i4} \partial_{i3} \sigma_{i1i1}) + (S_i^{i2} S^{i1i1} \partial_t \partial_t \sigma_{i1i2}) \right) + \right. \\ \left. 2 \left( (S_i^{i3} S_{i3}^{i4} v^i v^{i1} v^{i2} \partial_{i2} \partial_t \sigma_{i1i4}) - (S_i^{i3} S_{i3}^{i4} v^i v^{i1} v^{i2} \partial_{i4} \partial_t \sigma_{i1i2}) + \right. \right. \\ \left. \left. (S_i^{i2} S_{i2}^{i3} v^i v^{i1} \partial_t \partial_t \sigma_{i1i3}) \right) \right) \Big\}$$

$$\left\{ \begin{array}{c} \text{Diagram: A blue circle on a horizontal line with two blue lines diverging upwards from it.} \end{array} \right., \frac{1}{8} (c^{-1})^9 \left( (S^{i1i2} v^i \sigma_{i1}^{i3} \partial_i \sigma_{i2i3}) + \right.$$

$$\left. 2 (S^{i1i2} v^i \sigma_{i1}^{i3} \partial_{i2} \sigma_{i1i3}) - 2 (S^{i1i2} v^i \sigma_{i1}^{i3} \partial_{i3} \sigma_{i1i2}) + (S^{i1i1} \sigma_i^{i2} \partial_t \sigma_{i1i2}) \right) \Big\}$$

$$\left\{ \begin{array}{c} \text{Diagram: A blue circle on a horizontal line with a vertical dashed green line passing through its center.} \end{array} \right.,$$

$$(c^{-1})^2 m (A^i v_i) + \frac{1}{2} (c^{-1})^4 m (A^i v_i) (v_i v^i) + \frac{3}{8} (c^{-1})^6 m (A^i v_i) (v_i v^i)^2 + \frac{5}{16} (c^{-1})^8 m (A^i v_i) (v_i v^i)^3 \Big\}$$

$$\left\{ \begin{array}{c} \text{Diagram: A blue circle on a horizontal line with a vertical dashed green line passing through its center.} \end{array} \right.,$$

$$-\frac{1}{2} (c^{-1})^3 (S_{i1i1} \partial^{i1} A^i) + (c^{-1})^5 \left( \frac{3}{4} (S_{i1i2} v^i v^{i1} \partial_i A^{i2}) - \frac{3}{4} (S_{i1i2} v^i v^{i1} \partial^{i2} A_i) + (S_{i1i1} v^i \partial_t A^{i1}) \right) + \\ (c^{-1})^7 \left( - (A^i v_i) (a^i S_{i1i1} v^{i1}) + \right. \\ \left. \frac{1}{16} (v_i v^i) (7 (S_{i1i2} v^i v^{i1} \partial_i A^{i2}) - 7 (S_{i1i2} v^i v^{i1} \partial^{i2} A_i) + 8 (S_{i1i1} v^i \partial_t A^{i1})) \right) + \\ \frac{1}{32} (c^{-1})^9 (v_i v^i) (-48 (A^i v_i) (a^i S_{i1i1} v^{i1}) + \\ (v_i v^i) (11 (S_{i1i2} v^i v^{i1} \partial_i A^{i2}) - 11 (S_{i1i2} v^i v^{i1} \partial^{i2} A_i) + 12 (S_{i1i1} v^i \partial_t A^{i1}))) \Big\}$$

$$\left\{ \begin{array}{c} \text{Diagram: A blue square on a horizontal line with a vertical dashed green line passing through its center.} \end{array} \right.,$$

$$- \frac{C_{ES^2} (c^{-1})^6 \left( (S_i^{i2} S_{i1i2} \partial^{i1} \partial_t A^i) + (S_{i1}^{i3} S_{i2i3} v^i \partial^{i2} \partial_i A^{i1}) - (S_{i1}^{i3} S_{i2i3} v^i \partial^{i2} \partial^{i1} A_i) \right)}{2m} +$$

$$\frac{1}{4m} C_{ES^2} (c^{-1})^8 \left( (S_{i1}^{i3} S_{i2i3} v^i v^{i1} \partial_i \partial_t A^{i2}) - (S_i^{i3} S_{i3}^{i4} v^i v^{i1} v^{i2} \partial_{i2} \partial_{i1} A_{i4}) - \right. \\ (v_i v^i) \left( (S_i^{i2} S_{i1i2} \partial^{i1} \partial_t A^i) + (S_{i1}^{i3} S_{i2i3} v^i \partial^{i2} \partial_i A^{i1}) - (S_{i1}^{i3} S_{i2i3} v^i \partial^{i2} \partial^{i1} A_i) \right) + \\ (S_{i1}^{i3} S_{i2i3} v^i v^{i1} \partial^{i2} \partial_t A_i) - (S_{i2}^{i4} S_{i3i4} v^i v^{i1} v^{i2} \partial^{i3} \partial_{i1} A_i) + \\ \left. (S_i^{i3} S_{i1}^{i4} v^i v^{i1} v^{i2} \partial_{i4} \partial_{i2} A_{i3}) - (S_{i1i3} S_{i2i4} v^i v^{i1} v^{i2} \partial^{i4} \partial_i A^{i3}) \right) -$$

$$\frac{1}{16m} c_{ES^2} (c^{-1})^{10} \left( 2 \left( S_i^{i2} S_{i1i2} v^i v^{i1} \right) \left( v^i v^{i1} \partial_{i1} \partial_t A_i \right) + \right. \\ \left. 3 \left( v_i v^i \right)^2 \left( \left( S_i^{i2} S_{i1i2} \partial^{i1} \partial_t A^i \right) + \left( S_{i1}^{i3} S_{i2i3} v^i \partial^{i2} \partial_i A^{i1} \right) - \left( S_{i1}^{i3} S_{i2i3} v^i \partial^{i2} \partial^{i1} A_i \right) \right) + \right. \\ \left( v_i v^i \right) \left( -3 \left( S_{i1}^{i3} S_{i2i3} v^i v^{i1} \partial_i \partial_t A^{i2} \right) + 3 \left( S_i^{i3} S_{i3}^{i4} v^i v^{i1} v^{i2} \partial_{i2} \partial_{i1} A_{i4} \right) - \right. \\ \left. 3 \left( S_{i1}^{i3} S_{i2i3} v^i v^{i1} \partial^{i2} \partial_t A_i \right) + 3 \left( S_{i2}^{i4} S_{i3i4} v^i v^{i1} v^{i2} \partial^{i3} \partial_{i1} A_i \right) - \right. \\ \left. 5 \left( S_i^{i3} S_{i1}^{i4} v^i v^{i1} v^{i2} \partial_{i4} \partial_{i2} A_{i3} \right) - 2 \left( S_i^{i3} S_{i1}^{i4} v^i v^{i1} v^{i2} \partial_{i4} \partial_{i3} A_{i2} \right) + \right. \\ \left. 5 \left( S_{i1i3} S_{i2i4} v^i v^{i1} v^{i2} \partial^{i4} \partial_i A^{i3} \right) + 2 \left( S_{i1i3} S_{i2i4} v^i v^{i1} v^{i2} \partial^{i4} \partial^{i3} A_i \right) \right) \Bigg\}$$

$$\left\{ \begin{array}{c} \text{Diagram: A horizontal line with a blue circle vertex. A solid blue line goes up and to the right. A dashed green line goes up and to the left.} \end{array} \right\}, \frac{1}{2} (c^{-1})^8 m \left( A^i v_i \right) \left( v^i v^{i1} \sigma_{i1i} \right) \Bigg\}$$

$$\left\{ \begin{array}{c} \text{Diagram: A horizontal line with a blue oval vertex. A solid blue line goes up and to the right. A dashed green line goes up and to the left.} \end{array} \right\},$$

$$\frac{1}{4} (c^{-1})^7 \left( - \left( S_{i1}^{i2} \sigma_{i1i2} \partial^{i1} A^i \right) + \left( S_i^{i2} \sigma_{i1i2} \partial^{i1} A^i \right) \right) + \frac{1}{8} (c^{-1})^9 \left( -3 \left( S_{i2}^{i3} v^i v^{i1} \sigma_{i1i3} \partial_i A^{i2} \right) - \right. \\ \left. 3 \left( S_{i1}^{i3} v^i v^{i1} \sigma_{i2i3} \partial_i A^{i2} \right) + 3 \left( S_{i2}^{i3} v^i v^{i1} \sigma_{i1i3} \partial^{i2} A_i \right) + 3 \left( S_{i1}^{i3} v^i v^{i1} \sigma_{i2i3} \partial^{i2} A_i \right) - \right. \\ \left. 4 \left( S_{i1}^{i2} v^i \sigma_{i1i2} \partial_t A^{i1} \right) - 4 \left( S_i^{i2} v^i \sigma_{i1i2} \partial_t A^{i1} \right) + 4 \left( A^i S_i^{i2} v^{i1} \partial_t \sigma_{i1i2} \right) \right) \Bigg\}$$

$$\left\{ \begin{array}{c} \text{Diagram: A horizontal line with a blue square vertex. A solid blue line goes up and to the right. A dashed green line goes up and to the left.} \end{array} \right\}, -\frac{1}{4m} c_{ES^2} (c^{-1})^{10}$$

$$\left( \left( S_{i2}^{i4} S_{i2i3} v^i \partial_i A^{i1} \partial_{i1} \sigma_{i3i4} \right) - \left( S_{i2}^{i4} S_{i2i3} v^i \partial_{i1} \sigma_{i3i4} \partial^{i1} A_i \right) + \left( S_{i1}^{i2} S_{i2}^{i3} \sigma_{i1i3} \partial^{i1} \partial_t A^i \right) + \right. \\ \left( S_i^{i2} S_{i2}^{i3} \sigma_{i1i3} \partial^{i1} \partial_t A^i \right) - \left( S_{i2}^{i3} S_{i3}^{i4} v^i \partial_i \sigma_{i1i4} \partial^{i2} A^{i1} \right) + \left( S_{i1}^{i3} S_{i3}^{i4} v^i \partial_i \sigma_{i2i4} \partial^{i2} A^{i1} \right) + \right. \\ \left( S_{i2}^{i3} S_{i3}^{i4} v^i \partial_{i1} \sigma_{i1i4} \partial^{i2} A^{i1} \right) - \left( S_{i1}^{i3} S_{i3}^{i4} v^i \partial_{i2} \sigma_{i1i4} \partial^{i2} A^{i1} \right) + \right. \\ \left( S_{i2}^{i3} S_{i3}^{i4} v^i \sigma_{i1i4} \partial^{i2} \partial_i A^{i1} \right) - \left( S_{i1}^{i3} S_{i3}^{i4} v^i \sigma_{i2i4} \partial^{i2} \partial_i A^{i1} \right) - \right. \\ \left( S_{i2}^{i3} S_{i3}^{i4} v^i \sigma_{i1i4} \partial^{i2} \partial^{i1} A_i \right) - \left( S_{i1}^{i3} S_{i3}^{i4} v^i \sigma_{i2i4} \partial^{i2} \partial^{i1} A_i \right) - \right. \\ \left( S_{i2}^{i3} S_{i3}^{i4} v^i \partial^{i2} A^{i1} \partial_{i4} \sigma_{i1i1} \right) + \left( S_{i1}^{i3} S_{i3}^{i4} v^i \partial^{i2} A^{i1} \partial_{i4} \sigma_{i1i2} \right) - \right. \\ \left. 2 \left( S_{i2}^{i4} S_{i2i3} v^i \partial_i A^{i1} \partial_{i4} \sigma_{i1i3} \right) + 2 \left( S_{i2}^{i4} S_{i2i3} v^i \partial^{i1} A_i \partial_{i4} \sigma_{i1i3} \right) - \right. \\ \left. 2 \left( S_{i1}^{i3} S_{i1i2} v^i \sigma_{i2}^{i4} \partial_{i4} \partial_i A_{i3} \right) + \left( S_{i1}^{i3} S_{i1i2} \partial_i \sigma_{i2i3} \partial_t A^i \right) - \right. \\ \left. 2 \left( S_{i1}^{i3} S_{i1i2} \partial_{i3} \sigma_{i1i2} \partial_t A^i \right) - \left( S_{i1}^{i2} S_{i2}^{i3} \partial^{i1} A^i \partial_t \sigma_{i1i3} \right) + \left( S_i^{i2} S_{i2}^{i3} \partial^{i1} A^i \partial_t \sigma_{i1i3} \right) \Bigg\}$$

$$\left\{ \begin{array}{c} \text{Diagram: A horizontal line with a blue circle vertex. Two dashed green lines go up and to the left and up and to the right.} \end{array} \right\}, \frac{1}{2} (c^{-1})^8 m \left( A^i v_i \right)^2 \left( v_i v^i \right) \Bigg\}$$

$$\left\{ \begin{array}{c} \bullet \\ \diagup \quad \diagdown \\ \bullet \end{array} \right. , \frac{1}{2} (c^{-1})^7 \left( (A^i v_i) (S_{ii1} \partial^{i1} A^i) + (A^i S_{ii1} \partial_t A^{i1}) \right) + \frac{3}{4} (c^{-1})^9$$
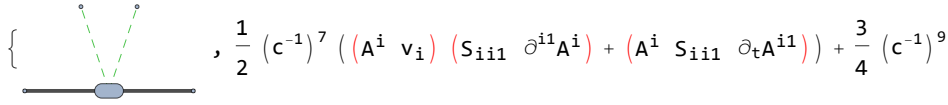

$$\left( (A^i S_{ii1} v^{i1}) (v^i \partial_t A_i) + (A^i v_i) \left( (S_{ii12} v^i v^{i1} \partial_i A^{i2}) - (S_{ii12} v^i v^{i1} \partial^{i2} A_i) + (S_{ii1} v^i \partial_t A^{i1}) \right) \right) \}$$

$$\left\{ \begin{array}{c} \bullet \\ \diagup \quad \diagdown \\ \bullet \end{array} \right. ,$$
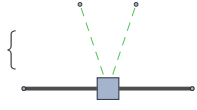

$$- \frac{C_{ES^2} (c^{-1})^8 \left( (S_i^{i3} S_{i2i3} \partial_{ii} A^{i2} \partial^{i1} A^i) + (S_{ii}^{i3} S_{i2i3} \partial^{i1} A^i \partial^{i2} A_i) - 2 (S_i^{i3} S_{i2i3} \partial^{i1} A^i \partial^{i2} A_{ii}) \right)}{8 m}$$

$$\begin{aligned} & - \frac{1}{16 m} C_{ES^2} (c^{-1})^{10} \left( 6 (S_{i2}^{i4} S_{i3i4} v^i v^{i1} \partial_i A^{i2} \partial_{ii} A^{i3}) + 8 (A^i S_i^{i3} S_{i2i3} v^{i1} \partial_{ii} \partial_t A^{i2}) + \right. \\ & (v_i v^i) (S_i^{i3} S_{i2i3} \partial_{ii} A^{i2} \partial^{i1} A^i) + 2 (S_{ii}^{i4} S_{i3i4} v^i v^{i1} \partial_i A^{i2} \partial_{i2} A^{i3}) - \\ & 12 (S_{i2}^{i4} S_{i3i4} v^i v^{i1} \partial_{ii} A^{i3} \partial^{i2} A_i) + (v_i v^i) (S_{ii}^{i3} S_{i2i3} \partial^{i1} A^i \partial^{i2} A_i) - \\ & 2 (S_{ii}^{i4} S_{i3i4} v^i v^{i1} \partial_{i2} A^{i3} \partial^{i2} A_i) - 2 (v_i v^i) (S_i^{i3} S_{i2i3} \partial^{i1} A^i \partial^{i2} A_{ii}) - \\ & 16 (A^i S_i^{i3} S_{i2i3} v^{i1} \partial^{i2} \partial_t A_{ii}) + 6 (S_{i2}^{i4} S_{i3i4} v^i v^{i1} \partial^{i2} A_i \partial^{i3} A_{ii}) - \\ & 2 (S_{ii}^{i4} S_{i3i4} v^i v^{i1} \partial_i A^{i2} \partial^{i3} A_{i2}) + 2 (S_{ii}^{i4} S_{i3i4} v^i v^{i1} \partial^{i2} A_i \partial^{i3} A_{i2}) - \\ & 8 (S_i^{i2} S_{ii12} \partial^{i1} A^i) (v^i \partial_t A_i) + 8 (S_i^{i2} S_{ii12} \partial_t A^i \partial_t A^{i1}) + 16 (S_{ii}^{i3} S_{i2i3} v^i \partial_i A^{i1} \partial_t A^{i2}) - \\ & \left. 8 (S_{ii}^{i3} S_{i2i3} v^i \partial^{i1} A_i \partial_t A^{i2}) + 8 (A^i S_i^{i2} S_{ii12} \partial_t \partial_t A^{i1}) \right) \} \end{aligned}$$

$$\left\{ \begin{array}{c} \bullet \\ | \\ \bullet \end{array} \right. , -m \phi + \frac{(c^{-1})^2 d m (v_i v^i) \phi}{4 - 2 d} +$$
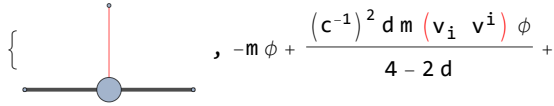

$$\frac{(c^{-1})^4 (2 - 3 d) m (v_i v^i)^2 \phi}{8 (-2 + d)} + \frac{(c^{-1})^6 (4 - 5 d) m (v_i v^i)^3 \phi}{16 (-2 + d)} - \frac{5 (c^{-1})^8 (-6 + 7 d) m (v_i v^i)^4 \phi}{128 (-2 + d)} \}$$

$$\left\{ \begin{array}{c} \bullet \\ | \\ \bullet \end{array} \right. ,$$
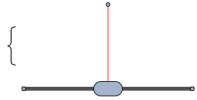

$$\begin{aligned} & (c^{-1})^3 \left( 1 + \frac{1}{-2 + d} \right) (S_{ii1} v^i \partial^{i1} \phi) + \frac{(c^{-1})^5 (-1 + d) \left( (v_i v^i) (S_{ii1} v^i \partial^{i1} \phi) + 2 (a^i S_{ii1} v^{i1}) \phi \right)}{2 (-2 + d)} + \\ & \frac{3 (c^{-1})^7 (-1 + d) (v_i v^i) \left( (v_i v^i) (S_{ii1} v^i \partial^{i1} \phi) + 4 (a^i S_{ii1} v^{i1}) \phi \right)}{8 (-2 + d)} + \\ & \frac{5 (c^{-1})^9 (-1 + d) (v_i v^i)^2 \left( (v_i v^i) (S_{ii1} v^i \partial^{i1} \phi) + 6 (a^i S_{ii1} v^{i1}) \phi \right)}{16 (-2 + d)} \} \end{aligned}$$

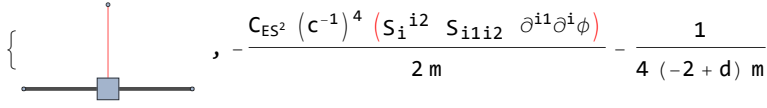

$$\left\{ , - \frac{C_{ES^2} (c^{-1})^4 (S_i^{i2} S_{i1i2} \partial^{i1} \partial^i \phi)}{2 m} - \frac{1}{4 (-2 + d) m} \right.$$

$$\begin{aligned} & C_{ES^2} (c^{-1})^6 (d (v_i v^i) (S_i^{i2} S_{i1i2} \partial^{i1} \partial^i \phi) - 4 (S_i^{i2} S_{i1i2} v^i \partial^{i1} \partial_t \phi) - 2 d (S_{i1}^{i3} S_{i2i3} v^i v^{i1} \partial^{i2} \partial_i \phi) + \\ & 2 (S_{i1i1} S^{ii1}) (2 (v^i \partial_i \partial_t \phi) + (v^i v^{i1} \partial_{i1} \partial_i \phi) + \partial_t \partial_t \phi)) + \frac{1}{32 (-2 + d) m} C_{ES^2} (c^{-1})^{10} (v_i v^i) \\ & ((v_i v^i) ((4 - 5 d) (v_i v^i) (S_i^{i2} S_{i1i2} \partial^{i1} \partial^i \phi) + 2 (-4 + 5 d) (S_{i1}^{i3} S_{i2i3} v^i v^{i1} \partial^{i2} \partial_i \phi) - \\ & 4 (-3 + 2 d) ((S_i^{i2} S_{i1}^{i3} v^i v^{i1} \partial_{i3} \partial_{i2} \phi) - (S_{i1i2} S_{i1i3} v^i v^{i1} \partial^{i3} \partial^{i2} \phi))) - \\ & 6 (S_{i1i1} S^{ii1}) (v_i v^i) (2 (v^i \partial_i \partial_t \phi) + (v^i v^{i1} \partial_{i1} \partial_i \phi) + \partial_t \partial_t \phi) + \\ & 4 (S_i^{i2} S_{i1i2} v^i v^{i1}) (3 (v^i \partial_i \partial_t \phi) - (-2 + d) (v^i v^{i1} \partial_{i1} \partial_i \phi) + 2 \partial_t \partial_t \phi)) + \frac{1}{16 (-2 + d) m} \\ & C_{ES^2} (c^{-1})^8 ((v_i v^i) ((2 - 3 d) (v_i v^i) (S_i^{i2} S_{i1i2} \partial^{i1} \partial^i \phi) + (-4 + 6 d) (S_{i1}^{i3} S_{i2i3} v^i v^{i1} \partial^{i2} \partial_i \phi) - \\ & 2 (-2 + d) ((S_i^{i2} S_{i1}^{i3} v^i v^{i1} \partial_{i3} \partial_{i2} \phi) - (S_{i1i2} S_{i1i3} v^i v^{i1} \partial^{i3} \partial^{i2} \phi))) - \\ & 4 (S_{i1i1} S^{ii1}) (v_i v^i) (2 (v^i \partial_i \partial_t \phi) + (v^i v^{i1} \partial_{i1} \partial_i \phi) + \partial_t \partial_t \phi) + \\ & (S_i^{i2} S_{i1i2} v^i v^{i1}) (8 (v^i \partial_i \partial_t \phi) - 2 (-2 + d) (v^i v^{i1} \partial_{i1} \partial_i \phi) + 8 \partial_t \partial_t \phi))) \} \end{aligned}$$

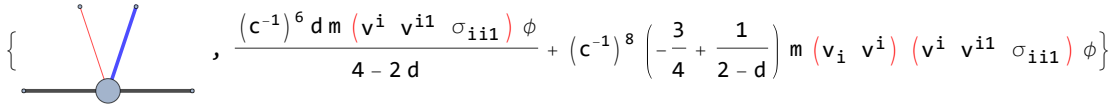

$$\left\{ , \frac{(c^{-1})^6 d m (v^i v^{i1} \sigma_{ii1}) \phi}{4 - 2 d} + (c^{-1})^8 \left( -\frac{3}{4} + \frac{1}{2 - d} \right) m (v_i v^i) (v^i v^{i1} \sigma_{ii1}) \phi \right\}$$

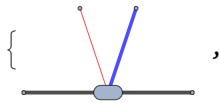

$$\left\{ , \right.$$

$$\begin{aligned} & - \frac{(c^{-1})^7 (-1 + d) ((S_{i1}^{i2} v^i \sigma_{ii2} \partial^{i1} \phi) + (S_i^{i2} v^i \sigma_{i1i2} \partial^{i1} \phi))}{2 (-2 + d)} + \frac{1}{4 (-2 + d)} (c^{-1})^9 (-1 + d) \\ & (2 (v^i v^{i1} \sigma_{ii1}) (S_{i1i1} v^i \partial^{i1} \phi) - (v_i v^i) ((S_{i1}^{i2} v^i \sigma_{ii2} \partial^{i1} \phi) + (S_i^{i2} v^i \sigma_{i1i2} \partial^{i1} \phi)) + \\ & 2 (-a^i S_{i1}^{i2} v^{i1} \sigma_{ii2}) + (a^i S_i^{i2} v^{i1} \sigma_{i1i2}) - 2 (S_i^{i3} v^i v^{i1} v^{i2} \partial_{i2} \sigma_{i1i3}) + \\ & (S_i^{i3} v^i v^{i1} v^{i2} \partial_{i3} \sigma_{i1i2}) - 3 (S_i^{i2} v^i v^{i1} \partial_t \sigma_{i1i2})) \phi) \} \end{aligned}$$

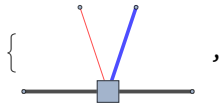

$$\left\{ , \right.$$

$$\begin{aligned} & - \frac{1}{4 m} C_{ES^2} (c^{-1})^8 ((S_{i1}^{i3} S_{i1i2} \partial_i \sigma_{i2i3} \partial^i \phi) + (S_{i1}^{i2} S_{i2}^{i3} \sigma_{ii3} \partial^{i1} \partial^i \phi) + (S_i^{i2} S_{i2}^{i3} \sigma_{i1i3} \partial^{i1} \partial^i \phi) - \\ & 2 (S_{i1}^{i3} S_{i1i2} \partial^i \phi \partial_{i3} \sigma_{i1i2})) + \\ & \frac{1}{8} C_{ES^2} (c^{-1})^{10} \left( \frac{d (v_i v^i) (S_{i1}^{i3} S_{i1i2} \partial_i \sigma_{i2i3} \partial^i \phi)}{2 m - d m} + \frac{2 d (v^i v^{i1} \sigma_{ii1}) (S_i^{i2} S_{i1i2} \partial^{i1} \partial^i \phi)}{2 m - d m} + \right. \\ & \left. \frac{d (v_i v^i) (S_{i1}^{i2} S_{i2}^{i3} \sigma_{ii3} \partial^{i1} \partial^i \phi)}{2 m - d m} + \frac{d (v_i v^i) (S_i^{i2} S_{i2}^{i3} \sigma_{i1i3} \partial^{i1} \partial^i \phi)}{2 m - d m} + \right. \end{aligned}$$

$$\begin{aligned}
& \frac{4 \left( S_{i1}^{i2} S_{i2}^{i3} v^i \sigma_{i1i3} \partial^{i1} \partial_t \phi \right)}{2m - dm} + \frac{4 \left( S_{i1}^{i2} S_{i2}^{i3} v^i \sigma_{i1i3} \partial^{i1} \partial_t \phi \right)}{(-2 + d)m} + \\
& \frac{4 \left( S_{i1i1} S^{ii1} \right) \left( v^i v^{i1} \partial_{i1} \sigma_{i1i2} \partial^{i2} \phi \right)}{(-2 + d)m} + \frac{2d \left( S_{i1}^{i3} S_{i3}^{i4} v^i v^{i1} \partial_{i1} \sigma_{i2i4} \partial^{i2} \phi \right)}{(-2 + d)m} + \\
& \frac{2 \left( S_{i1i1} S^{ii1} \right) \left( v^i v^{i1} \partial_{i2} \sigma_{i1i1} \partial^{i2} \phi \right)}{2m - dm} + \frac{2d \left( S_{i1}^{i3} S_{i3}^{i4} v^i v^{i1} \partial_{i2} \sigma_{i1i4} \partial^{i2} \phi \right)}{2m - dm} + \\
& \frac{2d \left( S_{i2}^{i3} S_{i3}^{i4} v^i v^{i1} \sigma_{i1i4} \partial^{i2} \partial_i \phi \right)}{2m - dm} + \frac{2d \left( S_{i1}^{i3} S_{i3}^{i4} v^i v^{i1} \sigma_{i2i4} \partial^{i2} \partial_i \phi \right)}{2m - dm} + \\
& \frac{2d \left( v_i v^i \right) \left( S_{i1}^{i3} S^{ii2} \partial^{i1} \phi \partial_{i3} \sigma_{i1i2} \right)}{(-2 + d)m} + \frac{\left( S_{i1i3} S_{i1}^{i4} v^i v^{i1} \sigma_{i2i4} \partial^{i3} \partial^{i2} \phi \right)}{m} + \\
& \frac{3 \left( S_{i1i2} S_{i1}^{i4} v^i v^{i1} \sigma_{i3i4} \partial^{i3} \partial^{i2} \phi \right)}{m} + \frac{2d \left( S_{i1}^{i3} S_{i3}^{i4} v^i v^{i1} \partial^{i2} \phi \partial_{i4} \sigma_{i1i2} \right)}{(-2 + d)m} + \\
& \frac{4d \left( S_{i1}^{i2} S_{i2}^{i3} v^i v^{i1} \sigma_{i3}^{i4} \partial_{i4} \partial_{i1} \phi \right)}{(-2 + d)m} - \frac{4 \left( S_{i1}^{i2} S_{i1}^{i3} v^i v^{i1} \sigma_{i2}^{i4} \partial_{i4} \partial_{i3} \phi \right)}{m} + \\
& \frac{4 \left( S_{i1i1} S^{ii1} \right) \left( v^i \partial^{i1} \phi \partial_t \sigma_{i1i1} \right)}{(-2 + d)m} - \frac{4(-1 + d) \left( S_{i1}^{i2} S_{i2}^{i3} v^i \partial^{i1} \phi \partial_t \sigma_{i1i3} \right)}{(-2 + d)m} - \\
& \frac{4(-1 + d) \left( v^i \partial_i \phi \right) \left( S_{i1}^{i2} S^{ii1} \partial_t \sigma_{i1i2} \right)}{(-2 + d)m} + \frac{4 \left( S_{i1}^{i2} S_{i2}^{i3} v^i \partial^{i1} \phi \partial_t \sigma_{i1i3} \right)}{(-2 + d)m} - \\
& \frac{4 \left( S_{i1}^{i3} S^{ii2} v^i \partial_i \partial_t \sigma_{i2i3} \right) \phi}{m} - \frac{2 \left( S_{i2}^{i4} S^{i2i3} v^i v^{i1} \partial_{i1} \partial_i \sigma_{i3i4} \right) \phi}{m} + \\
& \frac{4 \left( S_{i1}^{i3} S^{ii2} v^i \partial_{i3} \partial_t \sigma_{i1i2} \right) \phi}{m} + \frac{4 \left( S_{i2}^{i4} S^{i2i3} v^i v^{i1} \partial_{i4} \partial_{i1} \sigma_{i1i3} \right) \phi}{m} - \\
& \frac{2 \left( S_{i2}^{i4} S^{i2i3} v^i v^{i1} \partial_{i4} \partial_{i3} \sigma_{i1i1} \right) \phi}{m} - \frac{2 \left( S_{i1}^{i2} S^{ii1} \partial_t \partial_t \sigma_{i1i2} \right) \phi}{m} + \frac{2d \left( S_{i1}^{i2} S^{ii1} \partial_t \sigma_{i1i2} \right) \partial_t \phi}{2m - dm} \Bigg\}
\end{aligned}$$

$$\left\{ \begin{array}{c} \text{Diagram: A blue circle on a horizontal line with two lines (one red, one green) extending upwards from it.} \end{array} \right., \left( c^{-1} \right)^4 m \left( A^i v_i \right) \phi + \frac{\left( c^{-1} \right)^6 dm \left( A^i v_i \right) \left( v_i v^i \right) \phi}{4 - 2d} + \frac{\left( c^{-1} \right)^8 (6 - 9d) m \left( A^i v_i \right) \left( v_i v^i \right)^2 \phi}{8(-2 + d)} \Bigg\}$$

$$\left\{ \begin{array}{c} \text{Diagram: A blue oval on a horizontal line with two lines (one red, one green) extending upwards from it.} \end{array} \right., \left( c^{-1} \right)^5 \left( -1 + \frac{1}{2 - d} \right) \left( S_{i1i1} \partial^{i1} A^i \right) \phi - \frac{\left( c^{-1} \right)^7 (-1 + d) \left( A^i S_{i1i1} v^{i1} \right) \partial_t \phi}{-2 + d} +$$

$$\frac{1}{8(-2 + d)} \left( c^{-1} \right)^9 (-1 + d) \left( 8 \left( A^i v_i \right) \left( \left( v_i v^i \right) \left( S_{i1i1} v^i \partial^{i1} \phi \right) + 2 \left( a^i S_{i1i1} v^{i1} \right) \phi \right) - \left( v_i v^i \right) \right. \\
\left. \left( 7 \left( S_{i1i2} v^i v^{i1} \partial_i A^{i2} \right) \phi - 7 \left( S_{i1i2} v^i v^{i1} \partial^{i2} A_i \right) \phi + 8 \left( S_{i1i1} v^i \partial_t A^{i1} \right) \phi + 4 \left( A^i S_{i1i1} v^{i1} \right) \partial_t \phi \right) \right) \Bigg\}$$

$$\left\{ \begin{array}{c} \text{Diagram: A blue square on a horizontal line with two lines (one red, one green) extending upwards from it.} \end{array} \right., \frac{1}{2(-2 + d)m}$$

$$C_{ES^2} \left( c^{-1} \right)^8 \left( (-2 + d) \left( A^i v_i \right) \left( S_{i1}^{i2} S_{i1i2} \partial^{i1} \partial^i \phi \right) + 4 \left( A^i S_{i1}^{i2} S_{i1i2} \partial^{i1} \partial_t \phi \right) - 2d \left( A^i S_{i1}^{i2} S_{i1i2} \partial^{i1} \partial_t \phi \right) - \right. \\
\left. \left( S_{i1}^{i3} S_{i2i3} v^i \partial_{i1} \phi \partial^{i2} A^{i1} \right) + \left( S_{i1}^{i3} S_{i1i3} v^i \partial_{i2} \phi \partial^{i2} A^{i1} \right) + 3 \left( S_{i1}^{i3} S_{i2i3} v^i \partial_i A^{i1} \partial^{i2} \phi \right) - \right.$$

$$\begin{aligned}
& 3 d \left( S_{i1}^{i3} S_{i2i3} v^i \partial_i A^{i1} \partial^{i2} \phi \right) - 3 \left( S_{i1}^{i3} S_{i2i3} v^i \partial^{i1} A_i \partial^{i2} \phi \right) + 3 d \left( S_{i1}^{i3} S_{i2i3} v^i \partial^{i1} A_i \partial^{i2} \phi \right) + \\
& \left( S_{i1i1} S^{ii1} \right) \left( \left( v^i \partial_i A^{i1} \partial_{i1} \phi \right) - \left( v^i \partial_{i1} \phi \partial^{i1} A_i \right) + \left( \partial^i \phi \partial_t A_i \right) \right) + 2 \left( S_i^{i2} S_{i1i2} \partial^i \phi \partial_t A^{i1} \right) - \\
& 2 d \left( S_i^{i2} S_{i1i2} \partial^i \phi \partial_t A^{i1} \right) - d \left( S_i^{i2} S_{i1i2} \partial^{i1} \partial_t A^i \right) \phi - d \left( S_{i1}^{i3} S_{i2i3} v^i \partial^{i2} \partial_i A^{i1} \right) \phi + \\
& d \left( S_{i1}^{i3} S_{i2i3} v^i \partial^{i2} \partial^{i1} A_i \right) \phi + 2 \left( S_i^{i2} S_{i1i2} \partial^{i1} A^i \right) \partial_t \phi - d \left( S_i^{i2} S_{i1i2} \partial^{i1} A^i \right) \partial_t \phi + \\
& \frac{1}{4} C_{ES^2} (c^{-1})^{10} \left\{ \frac{3 (-1+d) \left( S_{i1}^{i3} S_{i2i3} v^i v^{i1} \partial_i A^{i2} \right) \left( v^i \partial_i \phi \right)}{(-2+d) m} - \frac{4 \left( S_{i1i1} S^{ii1} \right) \left( A^i v_i \right) \left( v^i \partial_i \partial_t \phi \right)}{(-2+d) m} + \right. \\
& \frac{2 d \left( A^i S_i^{i2} S_{i1i2} v^{i1} \right) \left( v^i \partial_i \partial_t \phi \right)}{(-2+d) m} + \frac{\left( S_{i1i1} S^{ii1} \right) \left( v_i v^i \right) \left( v^i \partial_i A^{i1} \partial_{i1} \phi \right)}{(-2+d) m} + \\
& \frac{\left( S_i^{i2} S_{i1i2} v^i v^{i1} \right) \left( v^i \partial_i A^{i1} \partial_{i1} \phi \right)}{2 m - d m} + \frac{2 \left( S_{i1i1} S^{ii1} \right) \left( A^i v_i \right) \left( v^i v^{i1} \partial_{i1} \partial_i \phi \right)}{2 m - d m} + \\
& \frac{\left( S_{i1i1} S^{ii1} \right) \left( v_i v^i \right) \left( v^i \partial_{i1} \phi \partial^{i1} A_i \right)}{2 m - d m} + \frac{\left( S_i^{i2} S_{i1i2} v^i v^{i1} \right) \left( v^i \partial_{i1} \phi \partial^{i1} A_i \right)}{(-2+d) m} + \\
& d \frac{\left( A^i v_i \right) \left( v_i v^i \right) \left( S_i^{i2} S_{i1i2} \partial^{i1} \partial^i \phi \right)}{2 m - d m} + \frac{2 d \left( v_i v^i \right) \left( A^i S_i^{i2} S_{i1i2} \partial^{i1} \partial_t \phi \right)}{2 m - d m} + \\
& \frac{2 d \left( A^i v_i \right) \left( S_i^{i2} S_{i1i2} v^i \partial^{i1} \partial_t \phi \right)}{(-2+d) m} - \frac{3 (-1+d) \left( v^i \partial_i \phi \right) \left( S_{i1}^{i3} S_{i2i3} v^i v^{i1} \partial^{i2} A_i \right)}{(-2+d) m} - \\
& \frac{3 (-1+d) \left( v_i v^i \right) \left( S_{i1}^{i3} S_{i2i3} v^i \partial_i A^{i1} \partial^{i2} \phi \right)}{(-2+d) m} + \frac{3 (-1+d) \left( v_i v^i \right) \left( S_{i1}^{i3} S_{i2i3} v^i \partial^{i1} A_i \partial^{i2} \phi \right)}{(-2+d) m} + \\
& \frac{2 d \left( A^i v_i \right) \left( S_{i1}^{i3} S_{i2i3} v^i v^{i1} \partial^{i2} \partial_i \phi \right)}{(-2+d) m} + \frac{2 (-1+d) \left( S_i^{i2} S_{i1i2} v^i \partial^{i1} \phi \right) \left( v^i \partial_t A_i \right)}{(-2+d) m} + \\
& \frac{\left( S_{i1i1} S^{ii1} \right) \left( v_i v^i \right) \left( \partial^i \phi \partial_t A_i \right)}{(-2+d) m} + \frac{2 \left( S_i^{i2} S_{i1i2} v^i v^{i1} \right) \left( \partial^i \phi \partial_t A_i \right)}{2 m - d m} + \\
& \frac{2 (-1+d) \left( v^i \partial_i \phi \right) \left( S_i^{i2} S_{i1i2} v^i \partial_t A^{i1} \right)}{(-2+d) m} - \frac{2 (-1+d) \left( v_i v^i \right) \left( S_i^{i2} S_{i1i2} \partial^i \phi \partial_t A^{i1} \right)}{(-2+d) m} - \\
& \frac{\left( S_{i1}^{i3} S_{i2i3} v^i v^{i1} \partial_i \partial_t A^{i2} \right) \phi}{m} + \frac{\left( v_i v^i \right) \left( S_i^{i2} S_{i1i2} \partial^{i1} \partial_t A^i \right) \phi}{m} + \\
& \frac{\left( S_i^{i3} S_{i3}^{i4} v^i v^{i1} v^{i2} \partial_{i2} \partial_{i1} A_{i4} \right) \phi}{m} + \frac{\left( v_i v^i \right) \left( S_{i1}^{i3} S_{i2i3} v^i \partial^{i2} \partial_i A^{i1} \right) \phi}{m} - \\
& \frac{\left( v_i v^i \right) \left( S_{i1}^{i3} S_{i2i3} v^i \partial^{i2} \partial^{i1} A_i \right) \phi}{m} - \frac{\left( S_{i1}^{i3} S_{i2i3} v^i v^{i1} \partial^{i2} \partial_t A_i \right) \phi}{m} + \\
& \frac{\left( S_{i2}^{i4} S_{i3i4} v^i v^{i1} v^{i2} \partial^{i3} \partial_{i1} A_i \right) \phi}{m} - \frac{\left( S_i^{i3} S_{i1}^{i4} v^i v^{i1} v^{i2} \partial_{i4} \partial_{i2} A_{i3} \right) \phi}{m} + \\
& \frac{\left( S_{i1i3} S_{i2i4} v^i v^{i1} v^{i2} \partial^{i4} \partial_i A^{i3} \right) \phi}{m} + \frac{d \left( S_{i1}^{i3} S_{i2i3} v^i v^{i1} \partial_i A^{i2} \right) \partial_t \phi}{(-2+d) m} + \\
& \frac{2 \left( S_{i1i1} S^{ii1} \right) \left( v^i v^{i1} \partial_{i1} A_i \right) \partial_t \phi}{2 m - d m} + \frac{d \left( v_i v^i \right) \left( S_i^{i2} S_{i1i2} \partial^{i1} A^i \right) \partial_t \phi}{2 m - d m} + \\
& \left. \frac{d \left( S_{i1}^{i3} S_{i2i3} v^i v^{i1} \partial^{i2} A_i \right) \partial_t \phi}{(-2+d) m} + \frac{2 \left( S_{i1i1} S^{ii1} \right) \left( A^i v_i \right) \partial_t \partial_t \phi}{2 m - d m} + \frac{4 \left( A^i S_i^{i2} S_{i1i2} v^{i1} \right) \partial_t \partial_t \phi}{(-2+d) m} \right\}
\end{aligned}$$

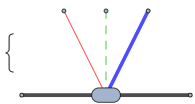

$$\left\{ , - \frac{(c^{-1})^9 (-1+d) \left( \left( S_{i1}^{i2} \sigma_{i1i2} \partial^{i1} A^i \right) - \left( S_i^{i2} \sigma_{i1i2} \partial^{i1} A^i \right) \right) \phi}{2 (-2+d)} \right\}$$

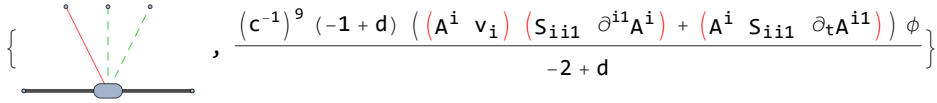

$$\left\{ , \frac{(c^{-1})^9 (-1+d) \left( (A^i v_i) (S_{ii1} \partial^{i1} A^i) + (A^i S_{ii1} \partial_t A^{i1}) \right) \phi}{-2+d} \right\}$$

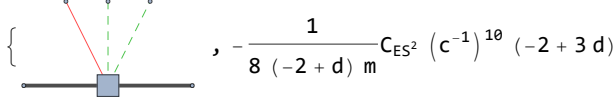

$$\left\{ , -\frac{1}{8(-2+d)m} C_{ES^2} (c^{-1})^{10} (-2+3d) \right\}$$

$$\left( (S_i^{i3} S_{i2i3} \partial_{i1} A^{i2} \partial^{i1} A^i) + (S_{i1}^{i3} S_{i2i3} \partial^{i1} A^i \partial^{i2} A_i) - 2 (S_i^{i3} S_{i2i3} \partial^{i1} A^i \partial^{i2} A_{i1}) \right) \phi \}$$

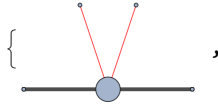

$$\left\{ , \right.$$

$$-\frac{1}{2} (c^{-1})^2 m \phi^2 + \frac{(c^{-1})^4 d^2 m (v_i v^i) \phi^2}{4(-2+d)^2} + \frac{(c^{-1})^6 (2-3d)^2 m (v_i v^i)^2 \phi^2}{16(-2+d)^2} + \frac{(c^{-1})^8 (4-5d)^2 m (v_i v^i)^3 \phi^2}{32(-2+d)^2} \}$$

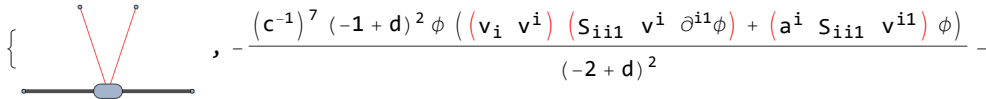

$$\left\{ , -\frac{(c^{-1})^7 (-1+d)^2 \phi \left( (v_i v^i) (S_{ii1} v^i \partial^{i1} \phi) + (a^i S_{ii1} v^{i1}) \phi \right)}{(-2+d)^2} - \right.$$

$$\left. \frac{3 (c^{-1})^9 (-1+d)^2 (v_i v^i) \phi \left( (v_i v^i) (S_{ii1} v^i \partial^{i1} \phi) + 2 (a^i S_{ii1} v^{i1}) \phi \right)}{2(-2+d)^2} \right\}$$

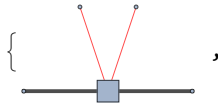

$$\left\{ , \right.$$

$$\begin{aligned} & \frac{C_{ES^2} (c^{-1})^6 \left( (S_{ii1} S^{ii1}) (\partial_i \phi \partial^i \phi) - d \left( (S_i^{i2} S_{i1i2} \partial^i \phi \partial^{i1} \phi) + (S_i^{i2} S_{i1i2} \partial^{i1} \partial^i \phi) \phi \right) \right)}{2(-2+d)m} + \\ & \frac{1}{4} C_{ES^2} (c^{-1})^8 \left( -\frac{2 (S_{ii1} S^{ii1}) (v^i \partial_i \phi)^2}{(-2+d)^2 m} + \frac{d (S_{ii1} S^{ii1}) (v_i v^i) (\partial_i \phi \partial^i \phi)}{(-2+d)^2 m} - \right. \\ & \frac{2(-1+d) (S_i^{i2} S_{i1i2} v^i v^{i1}) (\partial_i \phi \partial^i \phi)}{(-2+d)^2 m} + \frac{2(2-2d+d^2) (v^i \partial_i \phi) (S_i^{i2} S_{i1i2} v^i \partial^{i1} \phi)}{(-2+d)^2 m} - \\ & \frac{(2-2d+d^2) (v_i v^i) (S_i^{i2} S_{i1i2} \partial^i \phi \partial^{i1} \phi)}{(-2+d)^2 m} + \frac{2(-1+d) (S_{ii1} S^{ii1}) (\partial_t \phi)^2}{(-2+d)^2 m} + \\ & \frac{4 (S_{ii1} S^{ii1}) (v^i \partial_i \partial_t \phi) \phi}{(-2+d)m} + \frac{2 (S_{ii1} S^{ii1}) (v^i v^{i1} \partial_{i1} \partial_i \phi) \phi}{(-2+d)m} + \frac{d (v_i v^i) (S_i^{i2} S_{i1i2} \partial^{i1} \partial^i \phi) \phi}{(-2+d)m} - \\ & \left. \frac{4 (S_i^{i2} S_{i1i2} v^i \partial^{i1} \partial_t \phi) \phi}{(-2+d)m} + \frac{2d (S_{i1}^{i3} S_{i2i3} v^i v^{i1} \partial^{i2} \partial_i \phi) \phi}{2m-dm} + \frac{4 (S_{ii1} S^{ii1}) (v^i \partial_i \phi) \partial_t \phi}{(-2+d)m} - \right. \end{aligned}$$

$$\begin{aligned}
& \left. \frac{4 \left( S_i^{i2} S_{i1i2} v^i \partial^{i1} \phi \right) \partial_t \phi}{(-2+d) m} + \frac{2 \left( S_{ii1} S^{ii1} \right) \phi \partial_t \partial_t \phi}{(-2+d) m} \right\} + \frac{1}{16 (-2+d)^2 m} C_{ES^2} (c^{-1})^{10} \\
& \left( (v_i v^i) \left( 2 (4-6d+3d^2) (v^i \partial_i \phi) (S_i^{i2} S_{i1i2} v^i \partial^{i1} \phi) - 2 (-4+3d) ((-2+3d) (S_{i1}^{i3} S_{i2i3} v^i \right. \right. \\
& \quad \left. \left. v^{i1} \partial^{i2} \partial_i \phi) - (-2+d) ((S_i^{i2} S_{i1}^{i3} v^i v^{i1} \partial_{i3} \partial_{i2} \phi) - (S_{ii2} S_{i1i3} v^i v^{i1} \partial^{i3} \partial^{i2} \phi)) \right) \phi + \right. \\
& \quad (v_i v^i) \left( (-4+6d-3d^2) (S_i^{i2} S_{i1i2} \partial^i \phi \partial^{i1} \phi) + (8-18d+9d^2) (S_i^{i2} S_{i1i2} \partial^{i1} \partial^i \phi) \phi \right) - \\
& \quad 2 (S_i^{i2} S_{i1i2} v^i v^{i1}) \left( (-2+d) d (v^i \partial_i \phi)^2 + 2 (-1+d) (v_i v^i) (\partial_i \phi \partial^i \phi) - 8 (\partial_t \phi)^2 + \right. \\
& \quad \left. 4 d (\partial_t \phi)^2 - 16 (v^i \partial_i \partial_t \phi) \phi + 12 d (v^i \partial_i \partial_t \phi) \phi - 8 (v^i v^{i1} \partial_{i1} \partial_i \phi) \phi + 10 d (v^i v^{i1} \partial_{i1} \partial_i \phi) \phi - \right. \\
& \quad \left. 3 d^2 (v^i v^{i1} \partial_{i1} \partial_i \phi) \phi + 4 (-2+d) (v^i \partial_i \phi) \partial_t \phi - 16 \phi \partial_t \partial_t \phi + 12 d \phi \partial_t \partial_t \phi \right) + \\
& \quad (S_{ii1} S^{ii1}) (v_i v^i) \left( -4 (v^i \partial_i \phi)^2 + (-2+3d) (v_i v^i) (\partial_i \phi \partial^i \phi) + 4 (-3+d) (\partial_t \phi)^2 + \right. \\
& \quad \left. 8 (-2+d) (v^i \partial_i \phi) \partial_t \phi + 4 (-4+3d) \phi \left( 2 (v^i \partial_i \partial_t \phi) + (v^i v^{i1} \partial_{i1} \partial_i \phi) + \partial_t \partial_t \phi \right) \right) \Big\}
\end{aligned}$$

$$\left\{ \text{Diagram: A blue circle on a horizontal line with three lines (red, black, blue) extending upwards from its center.} \right\}, \frac{(c^{-1})^8 d^2 m (v^i v^{i1} \sigma_{ii1}) \phi^2}{4 (-2+d)^2}$$

$$\left\{ \text{Diagram: A blue square on a horizontal line with three lines (red, black, blue) extending upwards from its center.} \right\}, -\frac{1}{4 (-2+d) m} C_{ES^2} (c^{-1})^{10}$$

$$\begin{aligned}
& \left( 2 (S_{ii1} S^{ii1}) (\sigma_{ii1} \partial^i \phi \partial^{i1} \phi) + 2 d (S_i^{i2} S_{i2}^{i3} \sigma_{i1i3} \partial^i \phi \partial^{i1} \phi) + d ((S_{i1}^{i3} S^{i1i2} \partial_i \sigma_{i2i3} \partial^i \phi) + \right. \\
& \quad \left. (S_{i1}^{i2} S_{i2}^{i3} \sigma_{i1i3} \partial^{i1} \partial^i \phi) + (S_i^{i2} S_{i2}^{i3} \sigma_{i1i3} \partial^{i1} \partial^i \phi) - 2 (S_{i1}^{i3} S^{i1i2} \partial^i \phi \partial_{i3} \sigma_{ii2})) \phi \right\}
\end{aligned}$$

$$\left\{ \text{Diagram: A blue circle on a horizontal line with three lines (red, black, green) extending upwards from its center.} \right\}, \frac{1}{2} (c^{-1})^6 m (A^i v_i) \phi^2 + \frac{(c^{-1})^8 d^2 m (A^i v_i) (v_i v^i) \phi^2}{4 (-2+d)^2}$$

$$\left\{ \text{Diagram: A blue oval on a horizontal line with three lines (red, black, green) extending upwards from its center.} \right\}, -\frac{(c^{-1})^7 (-1+d)^2 (S_{ii1} \partial^{i1} A^i) \phi^2}{(-2+d)^2}$$

$$\left\{ \text{Diagram: A blue square on a horizontal line with three lines (red, black, green) extending upwards from its center.} \right\}, \frac{1}{4 (-2+d)^2 m}$$

$$\begin{aligned}
& C_{ES^2} (c^{-1})^{10} \left( 2 (S_{ii1} S^{ii1}) (-(-2+d) (A^i v_i) (\partial_i \phi \partial^i \phi) + d (v^i \partial_i A^{i1} \partial_{i1} \phi) \phi - \right. \\
& \quad d (v^i \partial_{i1} \phi \partial^{i1} A_i) \phi + d (\partial^i \phi \partial_t A_i) \phi - 4 (A^i \partial_i \phi) \partial_t \phi + 2 d (A^i \partial_i \phi) \partial_t \phi) + \\
& \quad d (-4 (-2+d) (A^i S_{i1i2} S_{i1i2} \partial^{i1} \partial_t \phi) \phi - 2 (S_i^{i3} S_{i2i3} v^i \partial_{i1} \phi \partial^{i2} A^{i1}) \phi + \\
& \quad 2 (S_i^{i3} S_{i1i3} v^i \partial_{i2} \phi \partial^{i2} A^{i1}) \phi + 6 (S_{i1}^{i3} S_{i2i3} v^i \partial_i A^{i1} \partial^{i2} \phi) \phi - \\
& \quad 6 d (S_{i1}^{i3} S_{i2i3} v^i \partial_i A^{i1} \partial^{i2} \phi) \phi - 6 (S_{i1}^{i3} S_{i2i3} v^i \partial^{i1} A_i \partial^{i2} \phi) \phi + \\
& \quad \left. 6 d (S_{i1}^{i3} S_{i2i3} v^i \partial^{i1} A_i \partial^{i2} \phi) \phi + 4 (S_i^{i2} S_{i1i2} \partial^i \phi \partial_t A^{i1}) \phi - 4 d (S_i^{i2} S_{i1i2} \partial^i \phi \partial_t A^{i1}) \phi - \right.
\end{aligned}$$

$$d \left( S_i^{i2} S_{i1i2} \partial^{i1} \partial_t A^i \right) \phi^2 - d \left( S_{i1}^{i3} S_{i2i3} v^i \partial^{i2} \partial_i A^{i1} \right) \phi^2 + d \left( S_{i1}^{i3} S_{i2i3} v^i \partial^{i2} \partial^{i1} A_i \right) \phi^2 +$$

$$2 (-2 + d) \left( A^i v_i \right) \left( \left( S_i^{i2} S_{i1i2} \partial^i \phi \partial^{i1} \phi \right) + \left( S_i^{i2} S_{i1i2} \partial^{i1} \partial^i \phi \right) \phi \right) + 8 \left( A^i S_i^{i2} S_{i1i2} \partial^{i1} \phi \right) \partial_t \phi -$$

$$4 d \left( A^i S_i^{i2} S_{i1i2} \partial^{i1} \phi \right) \partial_t \phi + 4 \left( S_i^{i2} S_{i1i2} \partial^{i1} A^i \right) \phi \partial_t \phi - 2 d \left( S_i^{i2} S_{i1i2} \partial^{i1} A^i \right) \phi \partial_t \phi \Big\}$$

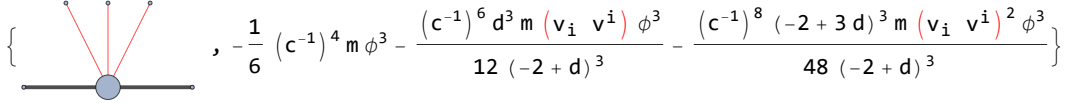

$$\left\{ , -\frac{1}{6} (c^{-1})^4 m \phi^3 - \frac{(c^{-1})^6 d^3 m (v_i v^i) \phi^3}{12 (-2 + d)^3} - \frac{(c^{-1})^8 (-2 + 3d)^3 m (v_i v^i)^2 \phi^3}{48 (-2 + d)^3} \right\}$$

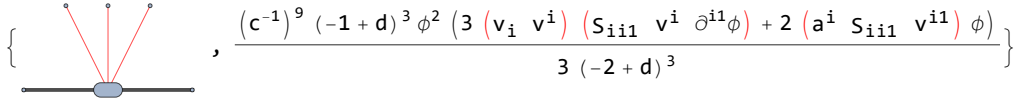

$$\left\{ , \frac{(c^{-1})^9 (-1 + d)^3 \phi^2 \left( 3 (v_i v^i) (S_{i1i1} v^i \partial^{i1} \phi) + 2 (a^i S_{i1i1} v^{i1}) \phi \right)}{3 (-2 + d)^3} \right\}$$

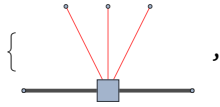

$$\left\{ , \right.$$

$$- \frac{C_{ES^2} (c^{-1})^8 d \phi \left( -2 (S_{i1i1} S^{i1i1}) (\partial_i \phi \partial^i \phi) + 2 d (S_i^{i2} S_{i1i2} \partial^i \phi \partial^{i1} \phi) + d (S_i^{i2} S_{i1i2} \partial^{i1} \partial^i \phi) \phi \right)}{4 (-2 + d)^2 m} +$$

$$\frac{1}{4} C_{ES^2} (c^{-1})^{10} \phi \left( \frac{2 (S_{i1i1} S^{i1i1}) (v^i \partial_i \phi)^2}{(-2 + d)^2 m} - \frac{d (S_{i1i1} S^{i1i1}) (v_i v^i) (\partial_i \phi \partial^i \phi)}{(-2 + d)^2 m} + \right.$$

$$\frac{2 (-1 + d) (S_i^{i2} S_{i1i2} v^i v^{i1}) (\partial_i \phi \partial^i \phi)}{(-2 + d)^2 m} - \frac{2 (2 - 2d + d^2) (v^i \partial_i \phi) (S_i^{i2} S_{i1i2} v^i \partial^{i1} \phi)}{(-2 + d)^2 m} +$$

$$\frac{(2 - 2d + d^2) (v_i v^i) (S_i^{i2} S_{i1i2} \partial^i \phi \partial^{i1} \phi)}{(-2 + d)^2 m} - \frac{2 (-1 + d) (S_{i1i1} S^{i1i1}) (\partial_t \phi)^2}{(-2 + d)^2 m} +$$

$$\frac{2 (S_{i1i1} S^{i1i1}) (v^i \partial_i \partial_t \phi) \phi}{2m - dm} + \frac{(S_{i1i1} S^{i1i1}) (v^i v^{i1} \partial_{i1} \partial_i \phi) \phi}{2m - dm} + \frac{d (v_i v^i) (S_i^{i2} S_{i1i2} \partial^{i1} \partial^i \phi) \phi}{4m - 2dm} +$$

$$\frac{2 (S_i^{i2} S_{i1i2} v^i \partial^{i1} \partial_t \phi) \phi}{(-2 + d)m} + \frac{d (S_{i1}^{i3} S_{i2i3} v^i v^{i1} \partial^{i2} \partial_i \phi) \phi}{(-2 + d)m} -$$

$$\left. \frac{4 (S_{i1i1} S^{i1i1}) (v^i \partial_i \phi) \partial_t \phi}{(-2 + d)m} + \frac{4 (S_i^{i2} S_{i1i2} v^i \partial^{i1} \phi) \partial_t \phi}{(-2 + d)m} + \frac{(S_{i1i1} S^{i1i1}) \phi \partial_t \partial_t \phi}{2m - dm} \right\}$$

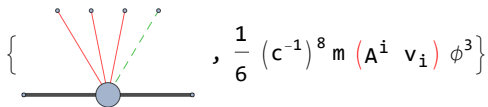

$$\left\{ , \frac{1}{6} (c^{-1})^8 m (A^i v_i) \phi^3 \right\}$$

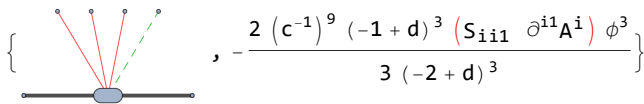

$$\left\{ , -\frac{2 (c^{-1})^9 (-1 + d)^3 (S_{i1i1} \partial^{i1} A^i) \phi^3}{3 (-2 + d)^3} \right\}$$

$$\left\{ \begin{array}{c} \text{Diagram: A horizontal line with a blue circle at its center. Five red lines radiate upwards from the circle to five small black dots arranged in a semi-circle above it.} \end{array} \right\}, -\frac{1}{24} (c^{-1})^6 m \phi^4 + \frac{(c^{-1})^8 d^4 m (v_i v^i) \phi^4}{48 (-2 + d)^4} \}$$

$$\left\{ \begin{array}{c} \text{Diagram: A horizontal line with a blue square at its center. Five red lines radiate upwards from the square to five small black dots arranged in a semi-circle above it.} \end{array} \right\},$$

$$-\frac{C_{ES^2} (c^{-1})^{10} d^2 \phi^2 \left( -3 (S_{i11} S^{i11}) (\partial_i \phi \partial^i \phi) + 3 d (S_i^{i2} S_{i1i2} \partial^i \phi \partial^{i1} \phi) + d (S_i^{i2} S_{i1i2} \partial^{i1} \partial^i \phi) \phi \right)}{12 (-2 + d)^3 m} \}$$

$$\left\{ \begin{array}{c} \text{Diagram: A horizontal line with a blue circle at its center. Five red lines radiate upwards from the circle to five small black dots arranged in a semi-circle above it.} \end{array} \right\}, -\frac{1}{120} (c^{-1})^8 m \phi^5 \}$$
