# Supplementary material for: N$^3$LO Quadratic-in-Spin Interactions for Generic Compact Binaries
Source: arXiv:2209.09235 ancillary file (2023-01-27)
Supplement: Supplementary file 2 [file graphs-CES1S1.pdf]

The diagram results are presented in MS-bar scheme.

Definitions :  $G = G_N$ ,  $\epsilon_d = d - 3$ ,  $\hat{n} = \frac{\vec{x}_1 - \vec{x}_2}{r}$ ,  $S_i^2 = \vec{S}_i^2$ ,  $\vec{A} = d^j \vec{A} / dt^j$

Legends :

- $\phi$  propagator
- - - A propagator
- $\sigma$  propagator
- worldlines
- mass coupling
- spin dipole coupling
- spin quadrupole coupling
- ★ time insertion

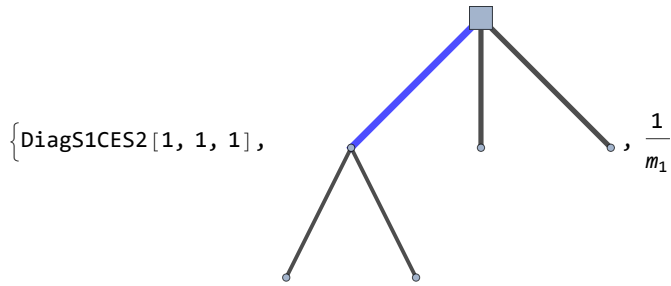

$$\begin{aligned}
 G \left( \frac{1}{r} \left( -2 \vec{v}_2 \cdot \vec{v}_2 \left( \frac{1}{S_1} \cdot \vec{v}_1 \right)^2 + 2 \vec{a}_1 \cdot \vec{v}_2 \vec{S}_1 \cdot \vec{v}_2 \frac{1}{S_1} \cdot \vec{v}_1 + 2 \frac{1}{S_1} \cdot \vec{v}_2 \vec{v}_1 \cdot \vec{v}_2 \frac{1}{S_1} \cdot \vec{v}_1 - 4 \vec{S}_1 \cdot \vec{a}_1 \vec{v}_2 \cdot \vec{v}_2 \frac{1}{S_1} \cdot \vec{v}_1 - \vec{a}_1 \cdot \vec{a}_1 \left( \vec{S}_1 \cdot \vec{v}_2 \right)^2 - \right. \right. \\
 2 \frac{1}{S_1} \cdot \vec{S}_1 \left( \vec{v}_1 \cdot \vec{v}_2 \right)^2 - 2 \vec{S}_1 \cdot \vec{S}_1 \left( \vec{v}_1 \cdot \vec{v}_2 \right)^2 - \frac{1}{S_1} \cdot \vec{S}_1 \left( \vec{v}_2 \cdot \vec{v}_2 \right)^2 - \vec{S}_1 \cdot \vec{S}_1 \left( \vec{v}_2 \cdot \vec{v}_2 \right)^2 - 2 \left( \vec{a}_1 \cdot \vec{v}_2 \right)^2 \vec{S}_1 \cdot \vec{S}_1 + \\
 2 \frac{1}{S_1} \cdot \vec{v}_2 \vec{a}_1 \cdot \vec{v}_2 \vec{S}_1 \cdot \vec{v}_1 + 2 \vec{a}_1 \cdot \vec{v}_2 \vec{S}_1 \cdot \vec{a}_1 \vec{S}_1 \cdot \vec{v}_2 + \frac{1}{\vec{a}_1} \cdot \vec{v}_2 \vec{S}_1 \cdot \vec{v}_1 \vec{S}_1 \cdot \vec{v}_2 - \left( \vec{S}_1 \cdot \vec{v}_2 \right)^2 \vec{v}_1 \cdot \vec{a}_1 - 4 \frac{1}{S_1} \cdot \vec{v}_2 \vec{S}_1 \cdot \vec{v}_2 \vec{v}_1 \cdot \vec{a}_1 - \\
 \left. \left( \frac{1}{S_1} \cdot \vec{v}_2 \right)^2 \vec{v}_1 \cdot \vec{v}_1 - \frac{2}{S_1} \cdot \vec{v}_2 \vec{S}_1 \cdot \vec{v}_2 \vec{v}_1 \cdot \vec{v}_1 - 8 \vec{a}_1 \cdot \vec{v}_2 \vec{S}_1 \cdot \vec{S}_1 \vec{v}_1 \cdot \vec{v}_2 + 2 \frac{1}{S_1} \cdot \vec{v}_2 \vec{S}_1 \cdot \vec{a}_1 \vec{v}_1 \cdot \vec{v}_2 - 2 \frac{1}{\vec{a}_1} \cdot \vec{v}_2 \vec{S}_1 \cdot \vec{S}_1 \vec{v}_1 \cdot \vec{v}_2 + \right. \\
 \frac{2}{S_1} \cdot \vec{v}_2 \vec{S}_1 \cdot \vec{v}_1 \vec{v}_1 \cdot \vec{v}_2 + 2 \frac{1}{S_1} \cdot \vec{a}_1 \vec{S}_1 \cdot \vec{v}_2 \vec{v}_1 \cdot \vec{v}_2 + \frac{2}{S_1} \cdot \vec{v}_1 \vec{S}_1 \cdot \vec{v}_2 \vec{v}_1 \cdot \vec{v}_2 + \vec{S}_1 \cdot \vec{a}_1 \vec{S}_1 \cdot \vec{v}_2 \vec{v}_1 \cdot \vec{v}_2 - \left. \left( \frac{1}{S_1} \cdot \vec{v}_2 \right)^2 \vec{v}_2 \cdot \vec{v}_2 - \right. \\
 2 \left( \vec{S}_1 \cdot \vec{a}_1 \right)^2 \vec{v}_2 \cdot \vec{v}_2 + \vec{a}_1 \cdot \vec{a}_1 \vec{S}_1 \cdot \vec{S}_1 \vec{v}_2 \cdot \vec{v}_2 - 4 \frac{1}{S_1} \cdot \vec{a}_1 \vec{S}_1 \cdot \vec{v}_1 \vec{v}_2 \cdot \vec{v}_2 - 2 \frac{2}{S_1} \cdot \vec{v}_1 \vec{S}_1 \cdot \vec{v}_1 \vec{v}_2 \cdot \vec{v}_2 - 2 \vec{S}_1 \cdot \frac{1}{\vec{a}_1} \vec{S}_1 \cdot \vec{v}_1 \vec{v}_2 \cdot \vec{v}_2 - \\
 \left. \frac{2}{S_1} \cdot \vec{v}_2 \vec{S}_1 \cdot \vec{v}_2 \vec{v}_2 \cdot \vec{v}_2 + \vec{S}_1 \cdot \vec{S}_1 \vec{v}_1 \cdot \frac{1}{\vec{a}_1} \vec{v}_2 \cdot \vec{v}_2 + 4 \vec{S}_1 \cdot \frac{1}{S_1} \vec{v}_1 \cdot \vec{a}_1 \vec{v}_2 \cdot \vec{v}_2 + \frac{1}{S_1} \cdot \vec{S}_1 \vec{v}_1 \cdot \vec{v}_1 \vec{v}_2 \cdot \vec{v}_2 + \vec{S}_1 \cdot \frac{2}{S_1} \vec{v}_1 \cdot \vec{v}_1 \vec{v}_2 \cdot \vec{v}_2 \right) + \\
 \frac{1}{r^2} \left( -\frac{1}{2} \hat{n} \cdot \vec{a}_1 \vec{v}_1 \cdot \vec{v}_1 \left( \vec{S}_1 \cdot \vec{v}_2 \right)^2 - \frac{1}{2} \hat{n} \cdot \vec{a}_1 \vec{v}_2 \cdot \vec{v}_2 \left( \vec{S}_1 \cdot \vec{v}_2 \right)^2 - \hat{n} \cdot \vec{v}_1 \vec{a}_1 \cdot \vec{v}_2 \vec{S}_1 \cdot \vec{v}_1 \vec{S}_1 \cdot \vec{v}_2 + \right. \\
 \hat{n} \cdot \vec{S}_1 \vec{a}_1 \cdot \vec{v}_2 \vec{v}_1 \cdot \vec{v}_1 \vec{S}_1 \cdot \vec{v}_2 - \hat{n} \cdot \vec{v}_1 \vec{S}_1 \cdot \vec{v}_1 \vec{v}_1 \cdot \vec{v}_2 \vec{S}_1 \cdot \vec{v}_2 - \hat{n} \cdot \vec{v}_1 \vec{S}_1 \cdot \vec{a}_1 \vec{v}_1 \cdot \vec{v}_2 \vec{S}_1 \cdot \vec{v}_2 + 2 \hat{n} \cdot \vec{S}_1 \vec{v}_1 \cdot \vec{a}_1 \vec{v}_1 \cdot \vec{v}_2 \vec{S}_1 \cdot \vec{v}_2 + \\
 \hat{n} \cdot \frac{1}{S_1} \vec{v}_1 \cdot \vec{v}_1 \vec{v}_1 \cdot \vec{v}_2 \vec{S}_1 \cdot \vec{v}_2 + \hat{n} \cdot \vec{S}_1 \vec{a}_1 \cdot \vec{v}_2 \vec{v}_2 \cdot \vec{v}_2 \vec{S}_1 \cdot \vec{v}_2 + \hat{n} \cdot \frac{1}{S_1} \vec{v}_1 \cdot \vec{v}_2 \vec{v}_2 \cdot \vec{v}_2 \vec{S}_1 \cdot \vec{v}_2 - \hat{n} \cdot \vec{S}_1 \vec{S}_1 \cdot \vec{v}_1 \left( \vec{v}_1 \cdot \vec{v}_2 \right)^2 + \\
 4 \hat{n} \cdot \vec{v}_1 \vec{S}_1 \cdot \frac{1}{S_1} \left( \vec{v}_1 \cdot \vec{v}_2 \right)^2 - \hat{n} \cdot \vec{S}_1 \vec{S}_1 \cdot \vec{a}_1 \left( \vec{v}_1 \cdot \vec{v}_2 \right)^2 + \hat{n} \cdot \vec{a}_1 \vec{S}_1 \cdot \vec{S}_1 \left( \vec{v}_1 \cdot \vec{v}_2 \right)^2 - \hat{n} \cdot \vec{S}_1 \vec{S}_1 \cdot \vec{v}_1 \left( \vec{v}_1 \cdot \vec{v}_2 \right)^2 - \\
 \hat{n} \cdot \vec{S}_1 \vec{S}_1 \cdot \vec{v}_1 \left( \vec{v}_2 \cdot \vec{v}_2 \right)^2 + 2 \hat{n} \cdot \vec{v}_1 \vec{S}_1 \cdot \frac{1}{S_1} \left( \vec{v}_2 \cdot \vec{v}_2 \right)^2 - \hat{n} \cdot \vec{S}_1 \vec{S}_1 \cdot \vec{a}_1 \left( \vec{v}_2 \cdot \vec{v}_2 \right)^2 + \frac{1}{2} \hat{n} \cdot \vec{a}_1 \vec{S}_1 \cdot \vec{S}_1 \left( \vec{v}_2 \cdot \vec{v}_2 \right)^2 - \\
 \hat{n} \cdot \vec{S}_1 \vec{S}_1 \cdot \vec{v}_1 \left( \vec{v}_2 \cdot \vec{v}_2 \right)^2 - \hat{n} \cdot \vec{v}_2 \vec{a}_1 \cdot \vec{v}_2 \vec{S}_1 \cdot \vec{S}_1 \vec{v}_1 \cdot \vec{v}_1 + 4 \hat{n} \cdot \vec{v}_1 \vec{a}_1 \cdot \vec{v}_2 \vec{S}_1 \cdot \vec{S}_1 \vec{v}_1 \cdot \vec{v}_2 - \hat{n} \cdot \vec{v}_1 \vec{S}_1 \cdot \vec{v}_2 \vec{S}_1 \cdot \vec{v}_1 \vec{v}_1 \cdot \vec{v}_2 - \\
 2 \hat{n} \cdot \vec{S}_1 \vec{a}_1 \cdot \vec{v}_2 \vec{S}_1 \cdot \vec{v}_1 \vec{v}_1 \cdot \vec{v}_2 - 2 \hat{n} \cdot \vec{v}_2 \vec{S}_1 \cdot \vec{S}_1 \vec{v}_1 \cdot \vec{a}_1 \vec{v}_1 \cdot \vec{v}_2 + \hat{n} \cdot \vec{S}_1 \frac{1}{S_1} \cdot \vec{v}_2 \vec{v}_1 \cdot \vec{v}_1 \vec{v}_1 \cdot \vec{v}_2 - \\
 2 \hat{n} \cdot \vec{v}_2 \vec{S}_1 \cdot \frac{1}{S_1} \vec{v}_1 \cdot \vec{v}_1 \vec{v}_1 \cdot \vec{v}_2 - \hat{n} \cdot \vec{v}_2 \vec{a}_1 \cdot \vec{v}_2 \vec{S}_1 \cdot \vec{S}_1 \vec{v}_2 \cdot \vec{v}_2 + 2 \hat{n} \cdot \vec{v}_1 \vec{S}_1 \cdot \vec{v}_1 \vec{S}_1 \cdot \vec{v}_1 \vec{v}_2 \cdot \vec{v}_2 + \\
 2 \hat{n} \cdot \vec{v}_1 \vec{S}_1 \cdot \vec{a}_1 \vec{S}_1 \cdot \vec{v}_1 \vec{v}_2 \cdot \vec{v}_2 - 2 \hat{n} \cdot \vec{v}_1 \vec{S}_1 \cdot \vec{S}_1 \vec{v}_1 \cdot \vec{a}_1 \vec{v}_2 \cdot \vec{v}_2 - 2 \hat{n} \cdot \vec{v}_1 \vec{S}_1 \cdot \frac{1}{S_1} \vec{v}_1 \cdot \vec{v}_1 \vec{v}_2 \cdot \vec{v}_2 -
 \end{aligned}$$

$$\begin{aligned} & \left( \frac{1}{2} \hat{n} \cdot \vec{a}_1 \vec{S}_1 \cdot \vec{S}_1 \vec{v}_1 \cdot \vec{v}_1 \vec{v}_2 \cdot \vec{v}_2 + \hat{n} \cdot \vec{S}_1 \vec{S}_1 \cdot \vec{v}_2 \vec{v}_1 \cdot \vec{v}_2 \vec{v}_2 \cdot \vec{v}_2 - 2 \hat{n} \cdot \vec{v}_2 \vec{S}_1 \cdot \vec{S}_1 \vec{v}_1 \cdot \vec{v}_2 \vec{v}_2 \cdot \vec{v}_2 \right) + \frac{1}{r^3} \\ & \left( -3 \vec{S}_1 \cdot \vec{S}_1 (\vec{v}_1 \cdot \vec{v}_2)^2 (\hat{n} \cdot \vec{v}_1)^2 + 3 \vec{S}_1 \cdot \vec{S}_1 \vec{v}_1 \cdot \vec{v}_1 \vec{v}_2 \cdot \vec{v}_2 (\hat{n} \cdot \vec{v}_1)^2 + 3 \hat{n} \cdot \vec{S}_1 \vec{S}_1 \cdot \vec{v}_1 (\vec{v}_1 \cdot \vec{v}_2)^2 \hat{n} \cdot \vec{v}_1 - \right. \\ & 3 \hat{n} \cdot \vec{S}_1 \vec{S}_1 \cdot \vec{v}_1 \vec{v}_1 \cdot \vec{v}_1 \vec{v}_2 \cdot \vec{v}_2 \hat{n} \cdot \vec{v}_1 - (\vec{S}_1 \cdot \vec{v}_1)^2 (\vec{v}_1 \cdot \vec{v}_2)^2 - \frac{3}{2} (\hat{n} \cdot \vec{S}_1)^2 \vec{v}_1 \cdot \vec{v}_1 (\vec{v}_1 \cdot \vec{v}_2)^2 + \\ & \frac{3}{2} \vec{S}_1 \cdot \vec{S}_1 \vec{v}_1 \cdot \vec{v}_1 (\vec{v}_1 \cdot \vec{v}_2)^2 + \frac{3}{2} (\hat{n} \cdot \vec{S}_1)^2 \vec{v}_1 \cdot \vec{v}_1 (\vec{v}_2 \cdot \vec{v}_2)^2 - \frac{1}{2} \vec{S}_1 \cdot \vec{S}_1 \vec{v}_1 \cdot \vec{v}_1 (\vec{v}_2 \cdot \vec{v}_2)^2 + \\ & \frac{3}{2} (\hat{n} \cdot \vec{S}_1)^2 (\vec{v}_1 \cdot \vec{v}_1)^2 \vec{v}_2 \cdot \vec{v}_2 - \frac{3}{2} \vec{S}_1 \cdot \vec{S}_1 (\vec{v}_1 \cdot \vec{v}_1)^2 \vec{v}_2 \cdot \vec{v}_2 - \frac{3}{2} (\hat{n} \cdot \vec{S}_1)^2 (\vec{v}_1 \cdot \vec{v}_2)^2 \vec{v}_2 \cdot \vec{v}_2 + \\ & \left. \frac{1}{2} \vec{S}_1 \cdot \vec{S}_1 (\vec{v}_1 \cdot \vec{v}_2)^2 \vec{v}_2 \cdot \vec{v}_2 + (\vec{S}_1 \cdot \vec{v}_1)^2 \vec{v}_1 \cdot \vec{v}_1 \vec{v}_2 \cdot \vec{v}_2 \right) \Big) m_2 C_{\text{ES}^2} \} \end{aligned}$$

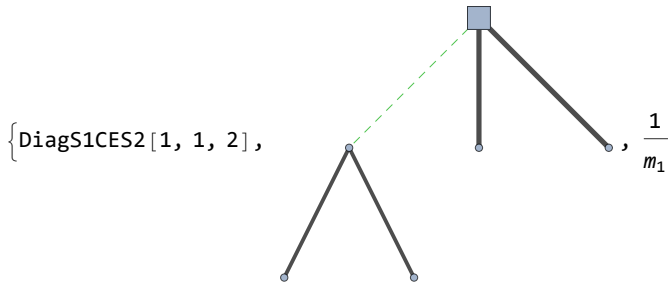

[illegible]

$$\left. \begin{aligned} & \frac{3}{4} \vec{S}_1 \cdot \vec{S}_1 \vec{v}_1 \cdot \vec{v}_2 (\vec{v}_2 \cdot \vec{v}_2)^2 + \frac{3}{2} (\hat{n} \cdot \vec{v}_1)^2 (\vec{S}_1 \cdot \vec{v}_1)^2 \vec{v}_1 \cdot \vec{v}_2 - \frac{7}{4} \vec{S}_1 \cdot \vec{S}_1 (\vec{v}_1 \cdot \vec{v}_1)^2 \vec{v}_1 \cdot \vec{v}_2 + \\ & (\vec{S}_1 \cdot \vec{v}_1)^2 \vec{v}_1 \cdot \vec{v}_1 \vec{v}_1 \cdot \vec{v}_2 + 3 (\hat{n} \cdot \vec{v}_1)^2 \vec{S}_1 \cdot \vec{S}_1 \vec{v}_1 \cdot \vec{v}_1 \vec{v}_1 \cdot \vec{v}_2 + (\vec{S}_1 \cdot \vec{v}_1)^2 \vec{v}_1 \cdot \vec{v}_2 \vec{v}_2 \cdot \vec{v}_2 + \\ & 3 (\hat{n} \cdot \vec{v}_1)^2 \vec{S}_1 \cdot \vec{S}_1 \vec{v}_1 \cdot \vec{v}_2 \vec{v}_2 \cdot \vec{v}_2 - \frac{3}{2} \vec{S}_1 \cdot \vec{S}_1 \vec{v}_1 \cdot \vec{v}_1 \vec{v}_1 \cdot \vec{v}_2 \vec{v}_2 \cdot \vec{v}_2 \end{aligned} \right) m_2 C_{ES^2_1} \}$$

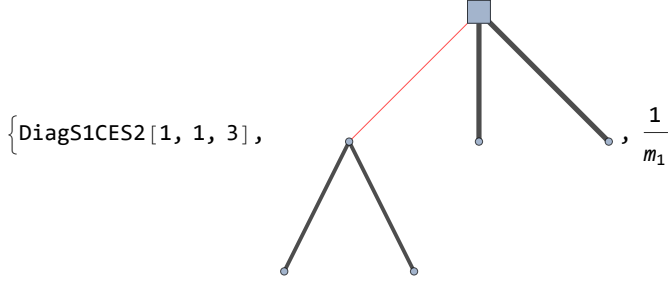

$$\begin{aligned} G \left( \frac{1}{r^2} \left( -\frac{1}{4} \hat{n} \cdot \vec{v}_1 \vec{v}_1 \cdot \vec{a}_1 (\vec{S}_1 \cdot \vec{v}_1)^2 + \frac{1}{8} \hat{n} \cdot \vec{a}_1 \vec{v}_1 \cdot \vec{v}_1 (\vec{S}_1 \cdot \vec{v}_1)^2 + \frac{7}{8} \hat{n} \cdot \vec{S}_1 (\vec{v}_2 \cdot \vec{v}_2)^2 \vec{S}_1 \cdot \vec{v}_1 - \frac{1}{4} \hat{n} \cdot \vec{v}_1 \vec{S}_1 \cdot \vec{v}_1 \vec{v}_1 \cdot \vec{v}_1 \vec{S}_1 \cdot \vec{v}_1 - \right. \right. \\ \left. \frac{1}{4} \hat{n} \cdot \vec{v}_1 \vec{S}_1 \cdot \vec{a}_1 \vec{v}_1 \cdot \vec{v}_1 \vec{S}_1 \cdot \vec{v}_1 - \frac{3}{2} \hat{n} \cdot \vec{v}_1 \vec{S}_1 \cdot \vec{v}_1 \vec{v}_2 \cdot \vec{v}_2 \vec{S}_1 \cdot \vec{v}_1 - \frac{3}{2} \hat{n} \cdot \vec{v}_1 \vec{S}_1 \cdot \vec{a}_1 \vec{v}_2 \cdot \vec{v}_2 \vec{S}_1 \cdot \vec{v}_1 + \right. \\ \left. \frac{1}{4} \hat{n} \cdot \vec{v}_1 \vec{S}_1 \cdot \vec{S}_1 (\vec{v}_1 \cdot \vec{v}_1)^2 + \frac{1}{4} \hat{n} \cdot \vec{a}_1 \vec{S}_1 \cdot \vec{S}_1 (\vec{v}_1 \cdot \vec{v}_1)^2 + \frac{7}{8} \hat{n} \cdot \vec{S}_1 \vec{S}_1 \cdot \vec{v}_1 (\vec{v}_2 \cdot \vec{v}_2)^2 - \right. \\ \left. \frac{7}{4} \hat{n} \cdot \vec{v}_1 \vec{S}_1 \cdot \vec{S}_1 (\vec{v}_2 \cdot \vec{v}_2)^2 + \frac{7}{8} \hat{n} \cdot \vec{S}_1 \vec{S}_1 \cdot \vec{a}_1 (\vec{v}_2 \cdot \vec{v}_2)^2 + \frac{1}{2} \hat{n} \cdot \vec{v}_1 \vec{S}_1 \cdot \vec{S}_1 \vec{v}_1 \cdot \vec{a}_1 \vec{v}_1 \cdot \vec{v}_1 + \right. \\ \left. \frac{3}{2} \hat{n} \cdot \vec{v}_1 \vec{S}_1 \cdot \vec{S}_1 \vec{v}_1 \cdot \vec{a}_1 \vec{v}_2 \cdot \vec{v}_2 + \frac{3}{2} \hat{n} \cdot \vec{v}_1 \vec{S}_1 \cdot \vec{S}_1 \vec{v}_1 \cdot \vec{v}_1 \vec{v}_2 \cdot \vec{v}_2 + \frac{3}{4} \hat{n} \cdot \vec{a}_1 \vec{S}_1 \cdot \vec{S}_1 \vec{v}_1 \cdot \vec{v}_1 \vec{v}_2 \cdot \vec{v}_2 \right) + \frac{1}{r^3} \\ \left( -\frac{33}{32} (\hat{n} \cdot \vec{S}_1)^2 (\vec{v}_1 \cdot \vec{v}_1)^3 + \frac{25}{32} \vec{S}_1 \cdot \vec{S}_1 (\vec{v}_1 \cdot \vec{v}_1)^3 - \frac{7}{16} (\vec{S}_1 \cdot \vec{v}_1)^2 (\vec{v}_1 \cdot \vec{v}_1)^2 - \frac{21}{16} (\hat{n} \cdot \vec{v}_1)^2 \vec{S}_1 \cdot \vec{S}_1 (\vec{v}_1 \cdot \vec{v}_1)^2 + \right. \\ \left. \frac{33}{16} \hat{n} \cdot \vec{S}_1 \hat{n} \cdot \vec{v}_1 \vec{S}_1 \cdot \vec{v}_1 (\vec{v}_1 \cdot \vec{v}_1)^2 - \frac{63}{32} (\hat{n} \cdot \vec{S}_1)^2 \vec{v}_2 \cdot \vec{v}_2 (\vec{v}_1 \cdot \vec{v}_1)^2 + \frac{57}{32} \vec{S}_1 \cdot \vec{S}_1 \vec{v}_2 \cdot \vec{v}_2 (\vec{v}_1 \cdot \vec{v}_1)^2 - \right. \\ \left. \frac{3}{4} (\hat{n} \cdot \vec{v}_1)^2 (\vec{S}_1 \cdot \vec{v}_1)^2 \vec{v}_1 \cdot \vec{v}_1 - \frac{63}{32} (\hat{n} \cdot \vec{S}_1)^2 (\vec{v}_2 \cdot \vec{v}_2)^2 \vec{v}_1 \cdot \vec{v}_1 + \frac{35}{32} \vec{S}_1 \cdot \vec{S}_1 (\vec{v}_2 \cdot \vec{v}_2)^2 \vec{v}_1 \cdot \vec{v}_1 - \right. \\ \left. \frac{9}{8} (\vec{S}_1 \cdot \vec{v}_1)^2 \vec{v}_2 \cdot \vec{v}_2 \vec{v}_1 \cdot \vec{v}_1 - \frac{27}{8} (\hat{n} \cdot \vec{v}_1)^2 \vec{S}_1 \cdot \vec{S}_1 \vec{v}_2 \cdot \vec{v}_2 \vec{v}_1 \cdot \vec{v}_1 + \frac{63}{16} \hat{n} \cdot \vec{S}_1 \hat{n} \cdot \vec{v}_1 \vec{S}_1 \cdot \vec{v}_1 \vec{v}_2 \cdot \vec{v}_2 \vec{v}_1 \cdot \vec{v}_1 - \right. \\ \left. \frac{33}{32} (\hat{n} \cdot \vec{S}_1)^2 (\vec{v}_2 \cdot \vec{v}_2)^3 + \frac{11}{32} \vec{S}_1 \cdot \vec{S}_1 (\vec{v}_2 \cdot \vec{v}_2)^3 - \frac{7}{16} (\vec{S}_1 \cdot \vec{v}_1)^2 (\vec{v}_2 \cdot \vec{v}_2)^2 - \right. \\ \left. \frac{21}{16} (\hat{n} \cdot \vec{v}_1)^2 \vec{S}_1 \cdot \vec{S}_1 (\vec{v}_2 \cdot \vec{v}_2)^2 + \frac{21}{16} \hat{n} \cdot \vec{S}_1 \hat{n} \cdot \vec{v}_1 \vec{S}_1 \cdot \vec{v}_1 (\vec{v}_2 \cdot \vec{v}_2)^2 - \frac{9}{16} (\hat{n} \cdot \vec{v}_1)^2 (\vec{S}_1 \cdot \vec{v}_1)^2 \vec{v}_2 \cdot \vec{v}_2 \right) + \\ \frac{1}{r} \left( \frac{1}{2} \vec{v}_1 \cdot \vec{v}_1 \left( \frac{1}{\vec{S}_1 \cdot \vec{v}_1} \right)^2 + \frac{3}{2} \vec{v}_2 \cdot \vec{v}_2 \left( \frac{1}{\vec{S}_1 \cdot \vec{v}_1} \right)^2 + 2 \vec{S}_1 \cdot \vec{v}_1 \vec{v}_1 \cdot \vec{a}_1 \vec{S}_1 \cdot \vec{v}_1 + \vec{S}_1 \cdot \vec{a}_1 \vec{v}_1 \cdot \vec{v}_1 \vec{S}_1 \cdot \vec{v}_1 + \right. \\ \left. 3 \vec{S}_1 \cdot \vec{a}_1 \vec{v}_2 \cdot \vec{v}_2 \vec{S}_1 \cdot \vec{v}_1 + \frac{1}{2} \vec{a}_1 \cdot \vec{a}_1 (\vec{S}_1 \cdot \vec{v}_1)^2 + \vec{S}_1 \cdot \vec{S}_1 (\vec{v}_1 \cdot \vec{a}_1)^2 - \frac{1}{2} \vec{S}_1 \cdot \vec{S}_1 (\vec{v}_1 \cdot \vec{v}_1)^2 - \frac{1}{2} \vec{S}_1 \cdot \vec{S}_1 (\vec{v}_1 \cdot \vec{v}_1)^2 + \right. \\ \left. \frac{1}{2} (\vec{S}_1 \cdot \vec{v}_1)^2 \vec{v}_1 \cdot \vec{a}_1 + 2 \vec{S}_1 \cdot \vec{a}_1 \vec{S}_1 \cdot \vec{v}_1 \vec{v}_1 \cdot \vec{a}_1 + \frac{1}{2} (\vec{S}_1 \cdot \vec{a}_1)^2 \vec{v}_1 \cdot \vec{v}_1 + \frac{1}{2} \vec{a}_1 \cdot \vec{a}_1 \vec{S}_1 \cdot \vec{S}_1 \vec{v}_1 \cdot \vec{v}_1 + \right. \\ \left. \frac{1}{\vec{S}_1 \cdot \vec{a}_1} \vec{S}_1 \cdot \vec{v}_1 \vec{v}_1 \cdot \vec{v}_1 + \frac{1}{2} \vec{S}_1 \cdot \vec{v}_1 \vec{S}_1 \cdot \vec{v}_1 \vec{v}_1 \cdot \vec{v}_1 + \frac{1}{2} \vec{S}_1 \cdot \vec{a}_1 \vec{S}_1 \cdot \vec{v}_1 \vec{v}_1 \cdot \vec{v}_1 + \frac{1}{2} \vec{S}_1 \cdot \vec{S}_1 \vec{v}_1 \cdot \vec{a}_1 \vec{v}_1 \cdot \vec{v}_1 - \right. \\ \left. 4 \vec{S}_1 \cdot \vec{S}_1 \vec{v}_1 \cdot \vec{a}_1 \vec{v}_1 \cdot \vec{v}_1 + \frac{3}{2} (\vec{S}_1 \cdot \vec{a}_1)^2 \vec{v}_2 \cdot \vec{v}_2 + 3 \vec{S}_1 \cdot \vec{a}_1 \vec{S}_1 \cdot \vec{v}_1 \vec{v}_2 \cdot \vec{v}_2 + \frac{3}{2} \vec{S}_1 \cdot \vec{v}_1 \vec{S}_1 \cdot \vec{v}_1 \vec{v}_2 \cdot \vec{v}_2 + \right. \\ \left. \frac{3}{2} \vec{S}_1 \cdot \vec{a}_1 \vec{S}_1 \cdot \vec{v}_1 \vec{v}_2 \cdot \vec{v}_2 - 6 \vec{S}_1 \cdot \vec{S}_1 \vec{v}_1 \cdot \vec{a}_1 \vec{v}_2 \cdot \vec{v}_2 - \frac{3}{2} \vec{S}_1 \cdot \vec{S}_1 \vec{v}_1 \cdot \vec{v}_1 \vec{v}_2 \cdot \vec{v}_2 - \frac{3}{2} \vec{S}_1 \cdot \vec{S}_1 \vec{v}_1 \cdot \vec{v}_1 \vec{v}_2 \cdot \vec{v}_2 + \right. \\ \left. 3 \vec{v}_1 \cdot \vec{a}_1 \vec{v}_1 \cdot \vec{v}_1 \vec{S}_1^2 + 3 \vec{v}_1 \cdot \vec{a}_1 \vec{v}_2 \cdot \vec{v}_2 \vec{S}_1^2 + \frac{3}{8} (\vec{v}_1 \cdot \vec{v}_1)^2 \vec{S}_1^2 + \frac{7}{8} (\vec{v}_2 \cdot \vec{v}_2)^2 \vec{S}_1^2 + \frac{3}{4} \vec{v}_1 \cdot \vec{v}_1 \vec{v}_2 \cdot \vec{v}_2 \vec{S}_1^2 \right) \Bigg) m_2 C_{ES^2_1} \} \end{aligned}$$

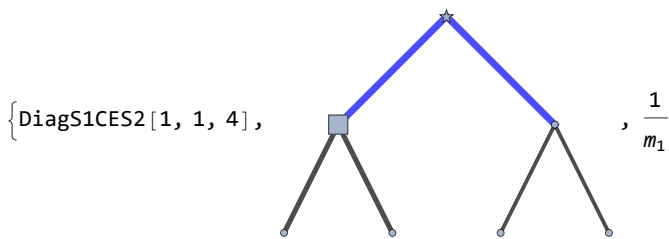

[illegible]

[illegible]

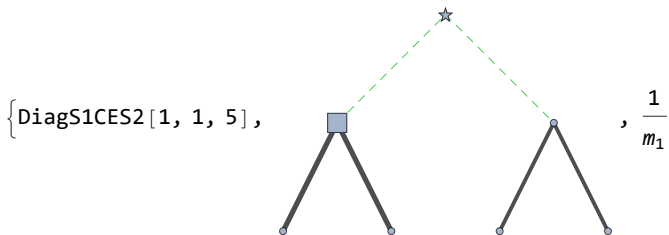

$$G \left( \hat{n} \cdot \overrightarrow{v_1} \overrightarrow{S_1}^{-1} \cdot \overrightarrow{a_2} \overrightarrow{S_1}^{-1} \cdot \overrightarrow{v_1} + \hat{n} \cdot \overrightarrow{S_1} \overrightarrow{a_1}^{-1} \cdot \overrightarrow{a_2} \overrightarrow{S_1}^{-1} \cdot \overrightarrow{v_1} + \hat{n} \cdot \overrightarrow{a_1} \overrightarrow{S_1}^{-1} \cdot \overrightarrow{a_2} \overrightarrow{S_1}^{-1} \cdot \overrightarrow{v_1} + \hat{n} \cdot \overrightarrow{S_1}^{-1} \overrightarrow{v_1}^{-1} \cdot \overrightarrow{a_2} \overrightarrow{S_1}^{-1} \cdot \overrightarrow{v_1} - 4 \hat{n} \cdot \overrightarrow{v_1} \overrightarrow{a_1}^{-1} \cdot \overrightarrow{a_2} \overrightarrow{S_1}^{-1} \cdot \overrightarrow{S_1}^{-1} + \right. \\ \left. \hat{n} \cdot \overrightarrow{v_1} \overrightarrow{S_1}^{-1} \cdot \overrightarrow{a_2} \overrightarrow{S_1}^{-1} \cdot \overrightarrow{a_1} + \hat{n} \cdot \overrightarrow{S_1}^{-1} \overrightarrow{a_1}^{-1} \cdot \overrightarrow{a_2} \overrightarrow{S_1}^{-1} \cdot \overrightarrow{a_1} + \hat{n} \cdot \overrightarrow{v_1} \overrightarrow{S_1}^{-1} \cdot \overrightarrow{a_1} \overrightarrow{S_1}^{-1} \cdot \overrightarrow{a_2} + \frac{1}{2} \hat{n} \cdot \overrightarrow{v_1} \overrightarrow{S_1}^{-1} \cdot \overrightarrow{v_1} \overrightarrow{S_1}^{-1} \cdot \overrightarrow{a_2} - \hat{n} \cdot \overrightarrow{S_1}^{-1} \overrightarrow{a_1}^{-1} \cdot \overrightarrow{a_1} \overrightarrow{S_1}^{-1} \cdot \overrightarrow{a_2} + \right.$$















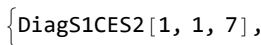

$$\begin{aligned}
G & \left( 3 \hat{n} \cdot \vec{v}_2 \vec{S}_1^{-1} \cdot \vec{a}_1 \vec{S}_1^{-1} \cdot \vec{v}_1 + \frac{3}{2} \hat{n} \cdot \vec{v}_2 \vec{S}_1^{-1} \cdot \vec{v}_1 \vec{S}_1^{-1} \cdot \vec{v}_1 + \frac{3}{2} \hat{n} \cdot \vec{v}_2 \vec{S}_1^{-1} \cdot \vec{a}_1 \vec{S}_1^{-1} \cdot \vec{v}_1 + 3 \hat{n} \cdot \vec{S}_1^{-1} \vec{v}_2 \cdot \vec{a}_2 \vec{S}_1^{-1} \cdot \vec{v}_1 - 3 \hat{n} \cdot \vec{v}_2 \vec{a}_1 \cdot \vec{a}_1 \vec{S}_1^{-1} \cdot \vec{S}_1^{-1} + \right. \\
& 3 \hat{n} \cdot \vec{v}_2 \vec{S}_1^{-1} \cdot \vec{a}_1 \vec{S}_1^{-1} \cdot \vec{a}_1 + \frac{3}{2} \hat{n} \cdot \vec{v}_2 \vec{S}_1^{-1} \cdot \vec{v}_1 \vec{S}_1^{-1} \cdot \vec{a}_1 + \frac{3}{2} \hat{n} \cdot \vec{v}_2 \vec{S}_1^{-1} \cdot \vec{a}_1 \vec{S}_1^{-1} \cdot \vec{a}_1 + \frac{3}{2} \hat{n} \cdot \vec{v}_2 \vec{S}_1^{-1} \cdot \vec{a}_1 \vec{S}_1^{-1} \cdot \vec{v}_1 + \\
& \frac{3}{2} \hat{n} \cdot \vec{v}_2 \vec{S}_1^{-1} \cdot \vec{a}_1 \vec{S}_1^{-1} \cdot \vec{v}_1 + \frac{1}{2} \hat{n} \cdot \vec{v}_2 \vec{S}_1^{-1} \cdot \vec{v}_1 \vec{S}_1^{-1} \cdot \vec{v}_1 + \frac{1}{2} \hat{n} \cdot \vec{v}_2 \vec{S}_1^{-1} \cdot \vec{a}_1 \vec{S}_1^{-1} \cdot \vec{v}_1 - 3 \hat{n} \cdot \vec{v}_2 \vec{S}_1^{-1} \cdot \vec{S}_1^{-1} \vec{v}_1 \cdot \vec{a}_1 - \\
& 3 \hat{n} \cdot \vec{v}_2 \vec{S}_1^{-1} \cdot \vec{S}_1^{-1} \vec{v}_1 \cdot \vec{a}_1 - 3 \hat{n} \cdot \vec{v}_2 \vec{S}_1^{-1} \cdot \vec{S}_1^{-1} \vec{v}_1 \cdot \vec{a}_1 - \frac{3}{2} \hat{n} \cdot \vec{v}_2 \vec{S}_1^{-1} \cdot \vec{S}_1^{-1} \vec{v}_1 \cdot \vec{v}_1 - \frac{1}{2} \hat{n} \cdot \vec{v}_2 \vec{S}_1^{-1} \cdot \vec{S}_1^{-1} \vec{v}_1 \cdot \vec{v}_1 - \\
& 3 \hat{n} \cdot \vec{v}_1 \vec{S}_1^{-1} \cdot \vec{S}_1^{-1} \vec{v}_2 \cdot \vec{a}_2 + 3 \hat{n} \cdot \vec{S}_1^{-1} \vec{S}_1^{-1} \cdot \vec{a}_1 \vec{v}_2 \cdot \vec{a}_2 + \frac{3}{2} \hat{n} \cdot \vec{S}_1^{-1} \vec{S}_1^{-1} \cdot \vec{v}_1 \vec{v}_2 \cdot \vec{a}_2 + \frac{3}{2} \hat{n} \cdot \vec{S}_1^{-1} \vec{S}_1^{-1} \cdot \vec{a}_1 \vec{v}_2 \cdot \vec{a}_2 - \\
& 6 \hat{n} \cdot \vec{a}_1 \vec{S}_1^{-1} \cdot \vec{S}_1^{-1} \vec{v}_2 \cdot \vec{a}_2 - 3 \hat{n} \cdot \vec{v}_1 \vec{S}_1^{-1} \cdot \vec{S}_1^{-1} \vec{v}_2 \cdot \vec{a}_2 + 3 \hat{n} \cdot \vec{S}_1^{-1} \vec{S}_1^{-1} \cdot \vec{a}_1 \vec{v}_2 \cdot \vec{a}_2 + \frac{3}{2} \hat{n} \cdot \vec{S}_1^{-1} \vec{S}_1^{-1} \cdot \vec{v}_1 \vec{v}_2 \cdot \vec{a}_2 + \frac{1}{r^2} \\
& \left( \frac{9}{4} \vec{S}_1^{-1} \cdot \vec{S}_1^{-1} \vec{v}_2 \cdot \vec{a}_2 \left( \hat{n} \cdot \vec{v}_1 \right)^3 + \frac{9}{8} \hat{n} \cdot \vec{v}_2 \vec{S}_1^{-1} \cdot \vec{v}_1 \vec{S}_1^{-1} \cdot \vec{v}_1 \left( \hat{n} \cdot \vec{v}_1 \right)^2 + \frac{9}{8} \hat{n} \cdot \vec{v}_2 \vec{S}_1^{-1} \cdot \vec{a}_1 \vec{S}_1^{-1} \cdot \vec{v}_1 \left( \hat{n} \cdot \vec{v}_1 \right)^2 - \right. \\
& \frac{15}{4} \hat{n} \cdot \vec{v}_2 \vec{S}_1^{-1} \cdot \vec{S}_1^{-1} \vec{v}_1 \cdot \vec{a}_1 \left( \hat{n} \cdot \vec{v}_1 \right)^2 - \frac{15}{4} \hat{n} \cdot \vec{v}_2 \vec{S}_1^{-1} \cdot \vec{S}_1^{-1} \vec{v}_1 \cdot \vec{v}_1 \left( \hat{n} \cdot \vec{v}_1 \right)^2 - \frac{9}{4} \hat{n} \cdot \vec{S}_1^{-1} \vec{S}_1^{-1} \cdot \vec{v}_1 \vec{v}_2 \cdot \vec{a}_2 \left( \hat{n} \cdot \vec{v}_1 \right)^2 + \\
& \frac{9}{4} \hat{n} \cdot \vec{v}_2 \vec{S}_1^{-1} \cdot \vec{S}_1^{-1} \vec{v}_2 \cdot \vec{v}_2 \left( \hat{n} \cdot \vec{v}_1 \right)^2 - \frac{3}{8} \hat{n} \cdot \vec{a}_1 \hat{n} \cdot \vec{v}_2 \left( \vec{S}_1^{-1} \cdot \vec{v}_1 \right)^2 \hat{n} \cdot \vec{v}_1 + \frac{1}{8} \vec{a}_1 \cdot \vec{v}_2 \left( \vec{S}_1^{-1} \cdot \vec{v}_1 \right)^2 \hat{n} \cdot \vec{v}_1 + \\
& \frac{21}{8} \hat{n} \cdot \vec{S}_1^{-1} \hat{n} \cdot \vec{v}_2 \vec{S}_1^{-1} \cdot \vec{v}_1 \vec{v}_1 \cdot \vec{a}_1 \hat{n} \cdot \vec{v}_1 - \frac{7}{8} \vec{S}_1^{-1} \cdot \vec{v}_1 \vec{S}_1^{-1} \cdot \vec{v}_2 \vec{v}_1 \cdot \vec{a}_1 \hat{n} \cdot \vec{v}_1 + \frac{21}{16} \hat{n} \cdot \vec{S}_1^{-1} \hat{n} \cdot \vec{v}_2 \vec{S}_1^{-1} \cdot \vec{v}_1 \vec{v}_1 \cdot \vec{v}_1 \hat{n} \cdot \vec{v}_1 + \\
& \left. \frac{21}{16} \hat{n} \cdot \vec{S}_1^{-1} \hat{n} \cdot \vec{v}_2 \vec{S}_1^{-1} \cdot \vec{a}_1 \vec{v}_1 \cdot \vec{v}_1 \hat{n} \cdot \vec{v}_1 - 3 \hat{n} \cdot \vec{a}_1 \hat{n} \cdot \vec{v}_2 \vec{S}_1^{-1} \cdot \vec{S}_1^{-1} \vec{v}_1 \cdot \vec{v}_1 \hat{n} \cdot \vec{v}_1 + \vec{a}_1 \cdot \vec{v}_2 \vec{S}_1^{-1} \cdot \vec{S}_1^{-1} \vec{v}_1 \cdot \vec{v}_1 \hat{n} \cdot \vec{v}_1 + \right.
\end{aligned}$$





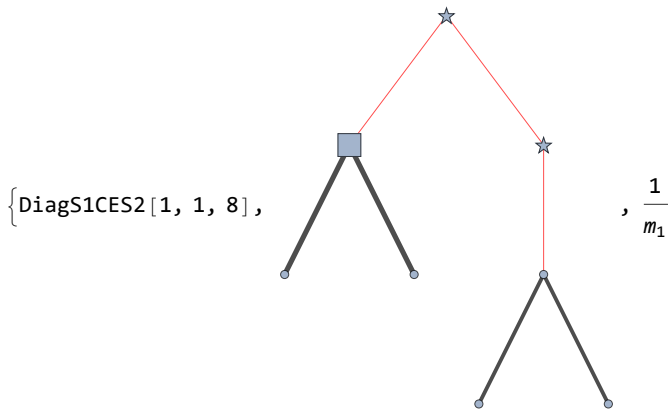

$$\begin{aligned}
G \left( -\frac{1}{8} \hat{n} \cdot \vec{a}_2 S_1^4 r^2 + \left( -\frac{3}{8} \vec{a}_2 \cdot \vec{a}_2 \left( \hat{n} \cdot \vec{S}_1 \right)^2 - \frac{3}{8} \vec{v}_2 \cdot \vec{a}_2 \left( \hat{n} \cdot \vec{S}_1 \right)^2 + \frac{3}{4} \hat{n} \cdot \vec{a}_2 \vec{S}_1 \cdot \vec{a}_1 \hat{n} \cdot \vec{S}_1 + \frac{3}{8} \hat{n} \cdot \vec{a}_2 \vec{S}_1 \cdot \vec{v}_1 \hat{n} \cdot \vec{S}_1 + \right. \right. \\
\frac{3}{8} \hat{n} \cdot \vec{a}_2 \vec{S}_1 \cdot \vec{a}_1 \hat{n} \cdot \vec{S}_1 + \frac{3}{8} \hat{n} \cdot \vec{a}_2 \hat{n} \cdot \vec{S}_1 \vec{S}_1 \cdot \vec{a}_1 - \frac{3}{4} \hat{n} \cdot \vec{a}_1 \hat{n} \cdot \vec{a}_2 \vec{S}_1 \cdot \vec{S}_1 - \frac{3}{4} \hat{n} \cdot \vec{a}_2 \hat{n} \cdot \vec{v}_1 \vec{S}_1 \cdot \vec{S}_1 + \\
\frac{3}{4} \vec{S}_1 \cdot \vec{a}_1 \vec{S}_1 \cdot \vec{a}_2 + \frac{3}{8} \hat{n} \cdot \vec{S}_1 \hat{n} \cdot \vec{a}_2 \vec{S}_1 \cdot \vec{v}_1 + \frac{3}{8} \hat{n} \cdot \vec{a}_2 \hat{n} \cdot \vec{S}_1 \vec{S}_1 \cdot \vec{a}_1 + \frac{3}{8} \vec{S}_1 \cdot \vec{v}_1 \vec{S}_1 \cdot \vec{a}_2 + \frac{3}{8} \vec{S}_1 \cdot \vec{a}_2 \vec{S}_1 \cdot \vec{v}_1 + \\
\frac{1}{8} \hat{n} \cdot \vec{a}_2 \hat{n} \cdot \vec{S}_1 \vec{S}_1 \cdot \vec{v}_1 - \frac{3}{4} \vec{S}_1 \cdot \vec{S}_1 \vec{a}_1 \cdot \vec{a}_2 - \frac{3}{8} \hat{n} \cdot \vec{S}_1 \hat{n} \cdot \vec{S}_1 \vec{a}_2 \cdot \vec{a}_2 + \frac{9}{8} \vec{S}_1 \cdot \vec{S}_1 \vec{a}_2 \cdot \vec{a}_2 + \frac{3}{8} \vec{S}_1 \cdot \vec{a}_2 \vec{S}_1 \cdot \vec{a}_1 + \\
\frac{1}{8} \hat{n} \cdot \vec{a}_2 \hat{n} \cdot \vec{S}_1 \vec{S}_1 \cdot \vec{a}_1 - \frac{3}{4} \hat{n} \cdot \vec{a}_1 \hat{n} \cdot \vec{a}_2 \vec{S}_1 \cdot \vec{S}_1 - \frac{3}{4} \vec{a}_1 \cdot \vec{a}_2 \vec{S}_1 \cdot \vec{S}_1 - \frac{3}{4} \hat{n} \cdot \vec{a}_1 \hat{n} \cdot \vec{a}_2 \vec{S}_1 \cdot \vec{S}_1 - \frac{3}{4} \vec{a}_1 \cdot \vec{a}_2 \vec{S}_1 \cdot \vec{S}_1 + \\
\frac{9}{8} \vec{a}_2 \cdot \vec{a}_2 \vec{S}_1 \cdot \vec{S}_1 - \frac{1}{4} \hat{n} \cdot \vec{a}_2 \hat{n} \cdot \vec{v}_1 \vec{S}_1 \cdot \vec{S}_1 + \frac{3}{8} \hat{n} \cdot \vec{S}_1 \hat{n} \cdot \vec{a}_2 \vec{S}_1 \cdot \vec{a}_1 + \frac{3}{8} \vec{S}_1 \cdot \vec{a}_2 \vec{S}_1 \cdot \vec{a}_1 + \frac{3}{8} \vec{S}_1 \cdot \vec{a}_1 \vec{S}_1 \cdot \vec{a}_2 + \\
\frac{3}{8} \vec{S}_1 \cdot \vec{a}_1 \vec{S}_1 \cdot \vec{a}_2 + \frac{1}{8} \vec{S}_1 \cdot \vec{v}_1 \vec{S}_1 \cdot \vec{a}_2 + \frac{1}{8} \vec{S}_1 \cdot \vec{a}_1 \vec{S}_1 \cdot \vec{a}_2 + \frac{1}{8} \hat{n} \cdot \vec{S}_1 \hat{n} \cdot \vec{a}_2 \vec{S}_1 \cdot \vec{v}_1 + \frac{1}{8} \vec{S}_1 \cdot \vec{a}_2 \vec{S}_1 \cdot \vec{v}_1 - \\
\frac{3}{4} \vec{S}_1 \cdot \vec{S}_1 \vec{v}_1 \cdot \vec{a}_2 - \frac{1}{4} \vec{S}_1 \cdot \vec{S}_1 \vec{v}_1 \cdot \vec{a}_2 - \frac{3}{8} \hat{n} \cdot \vec{S}_1 \hat{n} \cdot \vec{S}_1 \vec{v}_2 \cdot \vec{a}_2 + \frac{9}{8} \vec{S}_1 \cdot \vec{S}_1 \vec{v}_2 \cdot \vec{a}_2 + \frac{9}{8} \vec{S}_1 \cdot \vec{S}_1 \vec{v}_2 \cdot \vec{a}_2 + \\
\left. \frac{1}{4} \hat{n} \cdot \vec{a}_1 \hat{n} \cdot \vec{a}_2 S_1^2 + \frac{1}{4} \vec{a}_1 \cdot \vec{a}_2 S_1^2 - \frac{1}{4} \hat{n} \cdot \vec{a}_2 \hat{n} \cdot \vec{v}_1 S_1^2 - \frac{1}{4} \vec{v}_1 \cdot \vec{a}_2 S_1^2 + \frac{1}{8} (\hat{n} \cdot \vec{v}_2)^2 S_1^4 + \frac{1}{8} \vec{v}_2 \cdot \vec{v}_2 S_1^2 \right) r + \\
\frac{3}{8} \hat{n} \cdot \vec{a}_2 \left( \vec{S}_1 \cdot \vec{v}_1 \right)^2 + \frac{3}{8} \hat{n} \cdot \vec{S}_1 (\hat{n} \cdot \vec{v}_2)^2 \vec{S}_1 \cdot \vec{a}_1 + \frac{3}{8} \hat{n} \cdot \vec{a}_2 (\hat{n} \cdot \vec{v}_1)^2 \vec{S}_1 \cdot \vec{S}_1 - \frac{3}{4} \hat{n} \cdot \vec{a}_1 (\hat{n} \cdot \vec{v}_2)^2 \vec{S}_1 \cdot \vec{S}_1 - \\
\frac{3}{4} \hat{n} \cdot \vec{v}_1 (\hat{n} \cdot \vec{v}_2)^2 \vec{S}_1 \cdot \vec{S}_1 + \frac{3}{4} \hat{n} \cdot \vec{S}_1 (\hat{n} \cdot \vec{v}_2)^2 \vec{S}_1 \cdot \vec{a}_1 - \frac{3}{8} \hat{n} \cdot \vec{a}_2 \hat{n} \cdot \vec{S}_1 \hat{n} \cdot \vec{v}_1 \vec{S}_1 \cdot \vec{a}_1 + \\
\frac{3}{8} \hat{n} \cdot \vec{S}_1 (\hat{n} \cdot \vec{v}_2)^2 \vec{S}_1 \cdot \vec{v}_1 - \frac{3}{8} \hat{n} \cdot \vec{S}_1 \hat{n} \cdot \vec{a}_2 \hat{n} \cdot \vec{v}_1 \vec{S}_1 \cdot \vec{v}_1 + \frac{3}{8} \hat{n} \cdot \vec{v}_1 \vec{S}_1 \cdot \vec{a}_2 \vec{S}_1 \cdot \vec{v}_1 - \\
\frac{3}{2} \hat{n} \cdot \vec{v}_2 \vec{S}_1 \cdot \vec{a}_1 \vec{S}_1 \cdot \vec{v}_2 + \frac{3}{8} \hat{n} \cdot \vec{S}_1 (\hat{n} \cdot \vec{v}_2)^2 \vec{S}_1 \cdot \vec{a}_1 + \frac{3}{8} \hat{n} \cdot \vec{S}_1 (\hat{n} \cdot \vec{v}_2)^2 \vec{S}_1 \cdot \vec{v}_1 - \\
\frac{3}{16} \hat{n} \cdot \vec{a}_2 \hat{n} \cdot \vec{S}_1 \hat{n} \cdot \vec{v}_1 \vec{S}_1 \cdot \vec{v}_1 - \frac{3}{4} \hat{n} \cdot \vec{v}_2 \vec{S}_1 \cdot \vec{v}_2 \vec{S}_1 \cdot \vec{v}_1 - \frac{3}{4} \hat{n} \cdot \vec{v}_2 \vec{S}_1 \cdot \vec{v}_1 \vec{S}_1 \cdot \vec{v}_2 + \\
\frac{1}{8} \hat{n} \cdot \vec{S}_1 (\hat{n} \cdot \vec{v}_2)^2 \vec{S}_1 \cdot \vec{v}_1 - \frac{3}{16} \hat{n} \cdot \vec{a}_2 (\hat{n} \cdot \vec{S}_1)^2 \vec{a}_1 \cdot \vec{a}_1 + \frac{3}{2} \hat{n} \cdot \vec{v}_2 \vec{S}_1 \cdot \vec{S}_1 \vec{a}_1 \cdot \vec{v}_2 + \\
\frac{3}{16} \hat{n} \cdot \vec{a}_1 (\hat{n} \cdot \vec{S}_1)^2 \vec{a}_2 \cdot \vec{a}_2 + \frac{3}{4} \hat{n} \cdot \vec{S}_1 \hat{n} \cdot \vec{S}_1 \hat{n} \cdot \vec{v}_1 \vec{a}_2 \cdot \vec{a}_2 - \frac{3}{4} \hat{n} \cdot \vec{S}_1 \vec{S}_1 \cdot \vec{v}_1 \vec{a}_2 \cdot \vec{a}_2 + \\
\frac{3}{8} \hat{n} \cdot \vec{S}_1 (\hat{n} \cdot \vec{v}_2)^2 \vec{S}_1 \cdot \vec{a}_1 - \frac{3}{16} \hat{n} \cdot \vec{a}_2 \hat{n} \cdot \vec{S}_1 \hat{n} \cdot \vec{v}_1 \vec{S}_1 \cdot \vec{a}_1 - \frac{3}{4} \hat{n} \cdot \vec{v}_2 \vec{S}_1 \cdot \vec{v}_2 \vec{S}_1 \cdot \vec{a}_1 + \\
\frac{1}{8} \hat{n} \cdot \vec{S}_1 (\hat{n} \cdot \vec{v}_2)^2 \vec{S}_1 \cdot \vec{a}_1 - \frac{3}{4} \hat{n} \cdot \vec{a}_1 (\hat{n} \cdot \vec{v}_2)^2 \vec{S}_1 \cdot \vec{S}_1 + \frac{3}{4} \hat{n} \cdot \vec{a}_1 \hat{n} \cdot \vec{a}_2 \hat{n} \cdot \vec{v}_1 \vec{S}_1 \cdot \vec{S}_1 + \\
\frac{3}{2} \hat{n} \cdot \vec{v}_2 \vec{a}_1 \cdot \vec{v}_2 \vec{S}_1 \cdot \vec{S}_1 - \frac{3}{4} \hat{n} \cdot \vec{v}_1 \vec{a}_1 \cdot \vec{a}_2 \vec{S}_1 \cdot \vec{S}_1 + \frac{9}{4} \hat{n} \cdot \vec{v}_1 \vec{a}_2 \cdot \vec{a}_2 \vec{S}_1 \cdot \vec{S}_1 + \frac{3}{8} \hat{n} \cdot \vec{a}_2 (\hat{n} \cdot \vec{v}_1)^2 \vec{S}_1 \cdot \vec{S}_1 -
\end{aligned}$$

[illegible]











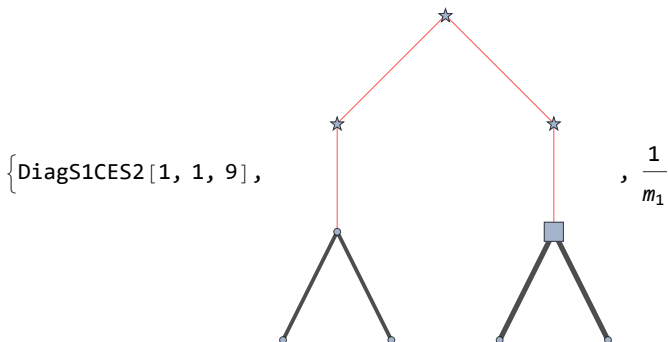

$$G \left( -\frac{3}{16} \hat{n} \cdot \overrightarrow{S_1} \hat{n} \cdot \overrightarrow{S_1} (\hat{n} \cdot \overrightarrow{v_2})^3 - \frac{1}{16} \hat{n} \cdot \overrightarrow{S_1} \hat{n} \cdot \overrightarrow{S_1} (\hat{n} \cdot \overrightarrow{v_2})^3 - \frac{5}{16} \overrightarrow{S_1} \cdot \overrightarrow{S_1} (\hat{n} \cdot \overrightarrow{v_2})^3 - \frac{5}{48} \overrightarrow{S_1} \cdot \overrightarrow{S_1} (\hat{n} \cdot \overrightarrow{v_2})^3 + \right. \\ \left. \frac{3}{16} \hat{n} \cdot \overrightarrow{S_1} \overrightarrow{S_1} \cdot \overrightarrow{v_2} (\hat{n} \cdot \overrightarrow{v_2})^2 + \frac{3}{16} \hat{n} \cdot \overrightarrow{S_1} \overrightarrow{S_1} \cdot \overrightarrow{v_2} (\hat{n} \cdot \overrightarrow{v_2})^2 + \frac{1}{16} \hat{n} \cdot \overrightarrow{S_1} \overrightarrow{S_1} \cdot \overrightarrow{v_2} (\hat{n} \cdot \overrightarrow{v_2})^2 + \frac{1}{16} \hat{n} \cdot \overrightarrow{S_1} \overrightarrow{S_1} \cdot \overrightarrow{v_2} (\hat{n} \cdot \overrightarrow{v_2})^2 + \right.$$















$$\begin{aligned}
& \frac{105}{16} \hat{n} \cdot \vec{S}_1 (\hat{n} \cdot \vec{v}_2)^2 \vec{S}_1 \cdot \vec{v}_2 (\hat{n} \cdot \vec{v}_1)^3 - \frac{105}{32} (\hat{n} \cdot \vec{S}_1)^2 \hat{n} \cdot \vec{v}_2 \vec{v}_2 \cdot \vec{v}_2 (\hat{n} \cdot \vec{v}_1)^3 - \\
& \frac{75}{32} \hat{n} \cdot \vec{v}_2 \vec{S}_1 \cdot \vec{S}_1 \vec{v}_2 \cdot \vec{v}_2 (\hat{n} \cdot \vec{v}_1)^3 + \frac{15}{16} \hat{n} \cdot \vec{S}_1 \vec{S}_1 \cdot \vec{v}_2 \vec{v}_2 \cdot \vec{v}_2 (\hat{n} \cdot \vec{v}_1)^3 - \frac{105}{16} \hat{n} \cdot \vec{S}_1 (\hat{n} \cdot \vec{v}_2)^3 \vec{S}_1 \cdot \vec{v}_1 (\hat{n} \cdot \vec{v}_1)^2 + \\
& \frac{45}{16} (\hat{n} \cdot \vec{v}_2)^2 \vec{S}_1 \cdot \vec{v}_1 \vec{S}_1 \cdot \vec{v}_2 (\hat{n} \cdot \vec{v}_1)^2 - \frac{315}{32} (\hat{n} \cdot \vec{S}_1)^2 (\hat{n} \cdot \vec{v}_2)^2 \vec{v}_1 \cdot \vec{v}_2 (\hat{n} \cdot \vec{v}_1)^2 - \\
& \frac{9}{16} (\vec{S}_1 \cdot \vec{v}_2)^2 \vec{v}_1 \cdot \vec{v}_2 (\hat{n} \cdot \vec{v}_1)^2 - \frac{225}{32} (\hat{n} \cdot \vec{v}_2)^2 \vec{S}_1 \cdot \vec{S}_1 \vec{v}_1 \cdot \vec{v}_2 (\hat{n} \cdot \vec{v}_1)^2 + \frac{45}{8} \hat{n} \cdot \vec{S}_1 \hat{n} \cdot \vec{v}_2 \vec{S}_1 \cdot \vec{v}_2 \vec{v}_1 \cdot \vec{v}_2 (\hat{n} \cdot \vec{v}_1)^2 + \\
& \frac{45}{16} \hat{n} \cdot \vec{S}_1 \hat{n} \cdot \vec{v}_2 \vec{S}_1 \cdot \vec{v}_1 \vec{v}_2 \cdot \vec{v}_2 (\hat{n} \cdot \vec{v}_1)^2 - \frac{9}{16} \vec{S}_1 \cdot \vec{v}_1 \vec{S}_1 \cdot \vec{v}_2 \vec{v}_2 \cdot \vec{v}_2 (\hat{n} \cdot \vec{v}_1)^2 + \frac{45}{32} (\hat{n} \cdot \vec{S}_1)^2 \vec{v}_1 \cdot \vec{v}_2 \vec{v}_2 \cdot \vec{v}_2 (\hat{n} \cdot \vec{v}_1)^2 + \\
& \frac{45}{32} \vec{S}_1 \cdot \vec{S}_1 \vec{v}_1 \cdot \vec{v}_2 \vec{v}_2 \cdot \vec{v}_2 (\hat{n} \cdot \vec{v}_1)^2 + \frac{15}{16} (\hat{n} \cdot \vec{v}_2)^3 (\vec{S}_1 \cdot \vec{v}_1)^2 \hat{n} \cdot \vec{v}_1 + \frac{45}{16} (\hat{n} \cdot \vec{S}_1)^2 \hat{n} \cdot \vec{v}_2 (\vec{v}_1 \cdot \vec{v}_2)^2 \hat{n} \cdot \vec{v}_1 + \\
& \frac{45}{16} \hat{n} \cdot \vec{v}_2 \vec{S}_1 \cdot \vec{S}_1 (\vec{v}_1 \cdot \vec{v}_2)^2 \hat{n} \cdot \vec{v}_1 - \frac{9}{8} \hat{n} \cdot \vec{S}_1 \vec{S}_1 \cdot \vec{v}_2 (\vec{v}_1 \cdot \vec{v}_2)^2 \hat{n} \cdot \vec{v}_1 - \frac{105}{32} (\hat{n} \cdot \vec{S}_1)^2 (\hat{n} \cdot \vec{v}_2)^3 \vec{v}_1 \cdot \vec{v}_1 \hat{n} \cdot \vec{v}_1 - \\
& \frac{9}{16} \hat{n} \cdot \vec{v}_2 (\vec{S}_1 \cdot \vec{v}_2)^2 \vec{v}_1 \cdot \vec{v}_1 \hat{n} \cdot \vec{v}_1 - \frac{75}{32} (\hat{n} \cdot \vec{v}_2)^3 \vec{S}_1 \cdot \vec{S}_1 \vec{v}_1 \cdot \vec{v}_1 \hat{n} \cdot \vec{v}_1 + \frac{45}{16} \hat{n} \cdot \vec{S}_1 (\hat{n} \cdot \vec{v}_2)^2 \vec{S}_1 \cdot \vec{v}_2 \vec{v}_1 \cdot \vec{v}_1 \hat{n} \cdot \vec{v}_1 + \\
& \frac{45}{8} \hat{n} \cdot \vec{S}_1 (\hat{n} \cdot \vec{v}_2)^2 \vec{S}_1 \cdot \vec{v}_1 \vec{v}_1 \cdot \vec{v}_2 \hat{n} \cdot \vec{v}_1 - \frac{9}{4} \hat{n} \cdot \vec{v}_2 \vec{S}_1 \cdot \vec{v}_1 \vec{S}_1 \cdot \vec{v}_2 \vec{v}_1 \cdot \vec{v}_2 \hat{n} \cdot \vec{v}_1 - \frac{9}{16} \hat{n} \cdot \vec{v}_2 (\vec{S}_1 \cdot \vec{v}_1)^2 \vec{v}_2 \cdot \vec{v}_2 \hat{n} \cdot \vec{v}_1 + \\
& \frac{45}{32} (\hat{n} \cdot \vec{S}_1)^2 \hat{n} \cdot \vec{v}_2 \vec{v}_1 \cdot \vec{v}_1 \vec{v}_2 \cdot \vec{v}_2 \hat{n} \cdot \vec{v}_1 + \frac{45}{32} \hat{n} \cdot \vec{v}_2 \vec{S}_1 \cdot \vec{S}_1 \vec{v}_1 \cdot \vec{v}_1 \vec{v}_2 \cdot \vec{v}_2 \hat{n} \cdot \vec{v}_1 - \\
& \frac{9}{16} \hat{n} \cdot \vec{S}_1 \vec{S}_1 \cdot \vec{v}_2 \vec{v}_1 \cdot \vec{v}_1 \vec{v}_2 \cdot \vec{v}_2 \hat{n} \cdot \vec{v}_1 - \frac{9}{8} \hat{n} \cdot \vec{S}_1 \vec{S}_1 \cdot \vec{v}_1 \vec{v}_1 \cdot \vec{v}_2 \vec{v}_2 \cdot \vec{v}_2 \hat{n} \cdot \vec{v}_1 - \frac{3}{16} (\hat{n} \cdot \vec{S}_1)^2 (\vec{v}_1 \cdot \vec{v}_2)^3 - \\
& \frac{5}{16} \vec{S}_1 \cdot \vec{S}_1 (\vec{v}_1 \cdot \vec{v}_2)^3 - \frac{9}{8} \hat{n} \cdot \vec{S}_1 \hat{n} \cdot \vec{v}_2 \vec{S}_1 \cdot \vec{v}_1 (\vec{v}_1 \cdot \vec{v}_2)^2 + \frac{3}{8} \vec{S}_1 \cdot \vec{v}_1 \vec{S}_1 \cdot \vec{v}_2 (\vec{v}_1 \cdot \vec{v}_2)^2 + \\
& \frac{15}{16} \hat{n} \cdot \vec{S}_1 (\hat{n} \cdot \vec{v}_2)^3 \vec{S}_1 \cdot \vec{v}_1 \vec{v}_1 \cdot \vec{v}_1 - \frac{9}{16} (\hat{n} \cdot \vec{v}_2)^2 \vec{S}_1 \cdot \vec{v}_1 \vec{S}_1 \cdot \vec{v}_2 \vec{v}_1 \cdot \vec{v}_1 - \frac{9}{16} (\hat{n} \cdot \vec{v}_2)^2 (\vec{S}_1 \cdot \vec{v}_1)^2 \vec{v}_1 \cdot \vec{v}_2 + \\
& \frac{45}{32} (\hat{n} \cdot \vec{S}_1)^2 (\hat{n} \cdot \vec{v}_2)^2 \vec{v}_1 \cdot \vec{v}_1 \vec{v}_1 \cdot \vec{v}_2 + \frac{3}{16} (\vec{S}_1 \cdot \vec{v}_2)^2 \vec{v}_1 \cdot \vec{v}_1 \vec{v}_1 \cdot \vec{v}_2 + \frac{45}{32} (\hat{n} \cdot \vec{v}_2)^2 \vec{S}_1 \cdot \vec{S}_1 \vec{v}_1 \cdot \vec{v}_1 \vec{v}_1 \cdot \vec{v}_2 - \\
& \frac{9}{8} \hat{n} \cdot \vec{S}_1 \hat{n} \cdot \vec{v}_2 \vec{S}_1 \cdot \vec{v}_2 \vec{v}_1 \cdot \vec{v}_1 \vec{v}_1 \cdot \vec{v}_2 - \frac{9}{16} \hat{n} \cdot \vec{S}_1 \hat{n} \cdot \vec{v}_2 \vec{S}_1 \cdot \vec{v}_1 \vec{v}_1 \cdot \vec{v}_1 \vec{v}_2 \cdot \vec{v}_2 + \frac{3}{16} \vec{S}_1 \cdot \vec{v}_1 \vec{S}_1 \cdot \vec{v}_2 \vec{v}_1 \cdot \vec{v}_1 \vec{v}_2 \cdot \vec{v}_2 + \\
& \frac{3}{16} (\vec{S}_1 \cdot \vec{v}_1)^2 \vec{v}_1 \cdot \vec{v}_2 \vec{v}_2 \cdot \vec{v}_2 - \frac{9}{32} (\hat{n} \cdot \vec{S}_1)^2 \vec{v}_1 \cdot \vec{v}_1 \vec{v}_1 \cdot \vec{v}_2 \vec{v}_2 \cdot \vec{v}_2 - \frac{15}{32} \vec{S}_1 \cdot \vec{S}_1 \vec{v}_1 \cdot \vec{v}_1 \vec{v}_1 \cdot \vec{v}_2 \vec{v}_2 \cdot \vec{v}_2 \Big) \Big) m_2 C_{ES^2 1} \Big\}
\end{aligned}$$

$\left\{ \text{DiagS1CES2}[2, 1, 1], \right.$ 
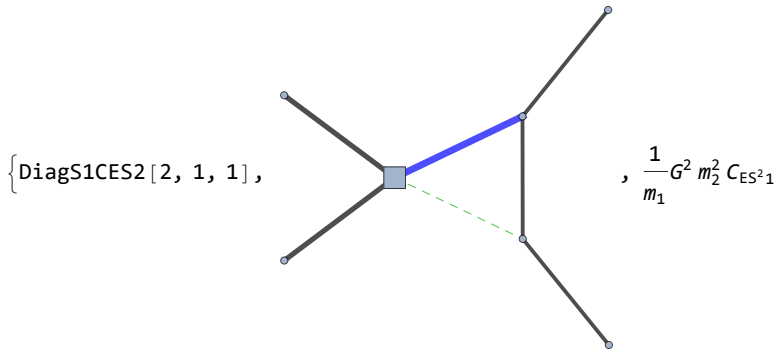
 $\left. , \frac{1}{m_1} G^2 m_2^2 C_{ES^2 1} \right\}$

$$\begin{aligned}
& \left( \frac{-8 \vec{S}_1 \cdot \vec{a}_2 \hat{n} \cdot \vec{v}_2 \vec{S}_1 \cdot \vec{v}_2 - 8 \vec{v}_2 \cdot \vec{a}_2 \hat{n} \cdot \vec{S}_1 \vec{S}_1 \cdot \vec{v}_2 + 16 \vec{S}_1 \cdot \vec{S}_1 \vec{v}_2 \cdot \vec{a}_2 \hat{n} \cdot \vec{v}_2 + 20 \vec{v}_2 \cdot \vec{v}_2 \vec{S}_1 \cdot \vec{a}_2 \hat{n} \cdot \vec{S}_1 - 12 \vec{S}_1 \cdot \vec{S}_1 \vec{v}_2 \cdot \vec{v}_2 \hat{n} \cdot \vec{a}_2}{r^3} \right. \\
& + \frac{1}{r^4} \left( 32 \vec{v}_1 \cdot \vec{v}_2 \vec{v}_2 \cdot \vec{v}_2 (\hat{n} \cdot \vec{S}_1)^2 - 24 \vec{v}_1 \cdot \vec{v}_2 \hat{n} \cdot \vec{S}_1 \hat{n} \cdot \vec{v}_2 \vec{S}_1 \cdot \vec{v}_2 - 4 \vec{v}_2 \cdot \vec{v}_2 \hat{n} \cdot \vec{S}_1 \hat{n} \cdot \vec{v}_2 \vec{S}_1 \cdot \vec{v}_1 - \right. \\
& 20 \vec{v}_2 \cdot \vec{v}_2 \hat{n} \cdot \vec{S}_1 \hat{n} \cdot \vec{v}_1 \vec{S}_1 \cdot \vec{v}_2 + 16 \vec{v}_2 \cdot \vec{v}_2 \hat{n} \cdot \vec{S}_1 \hat{n} \cdot \vec{v}_2 \vec{S}_1 \cdot \vec{v}_2 - 12 (\hat{n} \cdot \vec{v}_2)^2 (\vec{S}_1 \cdot \vec{v}_2)^2 + \\
& 12 \hat{n} \cdot \vec{v}_1 \hat{n} \cdot \vec{v}_2 (\vec{S}_1 \cdot \vec{v}_2)^2 + 24 \vec{S}_1 \cdot \vec{S}_1 \vec{v}_1 \cdot \vec{v}_2 (\hat{n} \cdot \vec{v}_2)^2 + 4 \vec{S}_1 \cdot \vec{S}_1 \vec{v}_2 \cdot \vec{v}_2 (\hat{n} \cdot \vec{v}_2)^2 + \\
& \left. \left. 4 \vec{S}_1 \cdot \vec{S}_1 \vec{v}_2 \cdot \vec{v}_2 \hat{n} \cdot \vec{v}_1 \hat{n} \cdot \vec{v}_2 + 4 \vec{v}_1 \cdot \vec{v}_2 (\vec{S}_1 \cdot \vec{v}_2)^2 + 8 \vec{v}_2 \cdot \vec{v}_2 \vec{S}_1 \cdot \vec{v}_1 \vec{S}_1 \cdot \vec{v}_2 - 20 \vec{S}_1 \cdot \vec{S}_1 \vec{v}_1 \cdot \vec{v}_2 \vec{v}_2 \cdot \vec{v}_2 \right) \right) \Big\}
\end{aligned}$$

{DiagS1CES2[2, 1, 2],

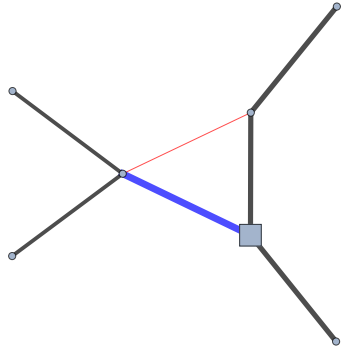

,

$$G^2 m_2 C_{ES^2 1} \left( \frac{1}{r^3} \left( -3 \hat{n} \cdot \vec{a}_1 (\vec{S}_1 \cdot \vec{v}_2)^2 + 6 \vec{a}_1 \cdot \vec{v}_2 \hat{n} \cdot \vec{S}_1 \vec{S}_1 \cdot \vec{v}_2 - 6 \vec{S}_1 \cdot \vec{S}_1 \vec{a}_1 \cdot \vec{v}_2 \hat{n} \cdot \vec{v}_2 - \right. \right. \\ \left. \left. 6 \vec{v}_2 \cdot \vec{v}_2 \vec{S}_1 \cdot \vec{a}_1 \hat{n} \cdot \vec{S}_1 + 3 \vec{S}_1 \cdot \vec{S}_1 \vec{v}_2 \cdot \vec{v}_2 \hat{n} \cdot \vec{a}_1 + 6 \vec{v}_1 \cdot \vec{v}_2 \hat{n} \cdot \vec{S}_1 \vec{S}_1 \cdot \vec{v}_2 + 6 \vec{v}_1 \cdot \vec{v}_2 \hat{n} \cdot \vec{S}_1 \vec{S}_1 \cdot \vec{v}_2 - \right. \right. \\ \left. \left. 12 \vec{S}_1 \cdot \vec{S}_1 \vec{v}_1 \cdot \vec{v}_2 \hat{n} \cdot \vec{v}_2 - 6 \vec{v}_2 \cdot \vec{v}_2 \hat{n} \cdot \vec{S}_1 \vec{S}_1 \cdot \vec{v}_1 + 12 \vec{S}_1 \cdot \vec{S}_1 \vec{v}_2 \cdot \vec{v}_2 \hat{n} \cdot \vec{v}_1 - 6 \vec{v}_2 \cdot \vec{v}_2 \hat{n} \cdot \vec{S}_1 \vec{S}_1 \cdot \vec{v}_1 \right) + \right. \\ \left. -9 (\vec{v}_1 \cdot \vec{v}_2)^2 (\hat{n} \cdot \vec{S}_1)^2 + 9 \vec{v}_1 \cdot \vec{v}_1 \vec{v}_2 \cdot \vec{v}_2 (\hat{n} \cdot \vec{S}_1)^2 + 3 \vec{S}_1 \cdot \vec{S}_1 (\vec{v}_1 \cdot \vec{v}_2)^2 - 3 \vec{S}_1 \cdot \vec{S}_1 \vec{v}_1 \cdot \vec{v}_1 \vec{v}_2 \cdot \vec{v}_2 \right) + \\ \left. \frac{-6 \left( \frac{1}{\vec{S}_1 \cdot \vec{v}_2} \right)^2 - 6 \frac{2}{\vec{S}_1 \cdot \vec{v}_2} \vec{S}_1 \cdot \vec{v}_2 - 6 \frac{1}{\vec{S}_1 \cdot \vec{S}_1} \vec{v}_2 \cdot \vec{v}_2 - 6 \vec{S}_1 \cdot \vec{S}_1 \vec{v}_2 \cdot \vec{v}_2}{r^2} \right\}$$

{DiagS1CES2[2, 1, 3],

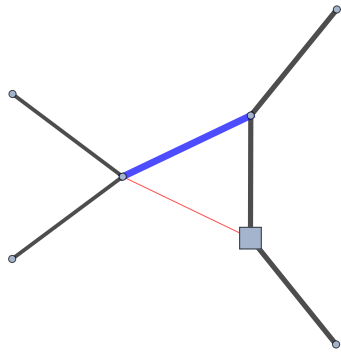

,

$$\frac{G^2 m_2 C_{ES^2 1} \left( -9 (\vec{v}_1 \cdot \vec{v}_2)^2 (\hat{n} \cdot \vec{S}_1)^2 + 9 \vec{v}_1 \cdot \vec{v}_1 \vec{v}_2 \cdot \vec{v}_2 (\hat{n} \cdot \vec{S}_1)^2 + 3 \vec{S}_1 \cdot \vec{S}_1 (\vec{v}_1 \cdot \vec{v}_2)^2 - 3 \vec{S}_1 \cdot \vec{S}_1 \vec{v}_1 \cdot \vec{v}_1 \vec{v}_2 \cdot \vec{v}_2 \right)}{r^4}$$

{DiagS1CES2[2, 1, 4],

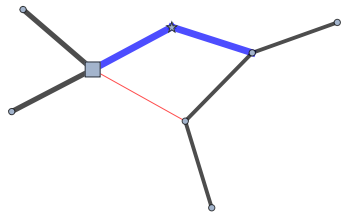

,  $\frac{1}{m_1}$

$$G^2 \left( \frac{1}{r^2} \left( -2 \hat{n} \cdot \vec{S}_1 \hat{n} \cdot \vec{v}_2 \vec{S}_1 \cdot \vec{a}_2 + \vec{S}_1 \cdot \vec{v}_2 \vec{S}_1 \cdot \vec{a}_2 - 2 \hat{n} \cdot \vec{a}_2 \hat{n} \cdot \vec{S}_1 \vec{S}_1 \cdot \vec{v}_2 + 8 \hat{n} \cdot \vec{a}_2 \hat{n} \cdot \vec{v}_2 \vec{S}_1 \cdot \vec{S}_1 - \right. \right. \\ \left. \left. 2 \hat{n} \cdot \vec{S}_1 \hat{n} \cdot \vec{v}_2 \vec{S}_1 \cdot \vec{a}_2 + \vec{S}_1 \cdot \vec{v}_2 \vec{S}_1 \cdot \vec{a}_2 - 2 \hat{n} \cdot \vec{S}_1 \hat{n} \cdot \vec{a}_2 \vec{S}_1 \cdot \vec{v}_2 + 8 \hat{n} \cdot \vec{S}_1 \hat{n} \cdot \vec{S}_1 \vec{v}_2 \cdot \vec{a}_2 - 6 \vec{S}_1 \cdot \vec{S}_1 \vec{v}_2 \cdot \vec{a}_2 \right) + \frac{1}{r^3} \right)$$

$$4 \hat{n} \cdot \vec{S}_1 \hat{n} \cdot \vec{v}_1 \vec{S}_1 \cdot \vec{v}_2 \vec{v}_2 \cdot \vec{v}_2 + \vec{S}_1 \cdot \vec{v}_1 \vec{S}_1 \cdot \vec{v}_2 \vec{v}_2 \cdot \vec{v}_2 - 4 \left( \hat{n} \cdot \vec{S}_1 \right)^2 \vec{v}_1 \cdot \vec{v}_2 \vec{v}_2 \cdot \vec{v}_2 + 3 \vec{S}_1 \cdot \vec{S}_1 \vec{v}_1 \cdot \vec{v}_2 \vec{v}_2 \cdot \vec{v}_2 \Big) m_D^2 C_{\text{ES}^2} \Big\}$$

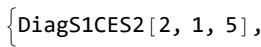

$$\begin{aligned} G^2 \left( \frac{1}{\rho^2} \right. & \left( 4 \vec{S}_1 \cdot \vec{S}_1 \left( \hat{n} \cdot \vec{a}_2 \right)^2 - 2 \hat{n} \cdot \vec{S}_1 \vec{S}_1 \cdot \vec{v}_2 \hat{n} \cdot \vec{a}_2 + 8 \hat{n} \cdot \vec{v}_2 \vec{S}_1 \cdot \vec{S}_1 \hat{n} \cdot \vec{a}_2 - 4 \hat{n} \cdot \vec{S}_1 \vec{S}_1 \cdot \vec{a}_2 \hat{n} \cdot \vec{a}_2 - \right. \\ & 2 \hat{n} \cdot \vec{S}_1 \vec{S}_1 \cdot \vec{v}_2 \hat{n} \cdot \vec{a}_2 + 2 \left( \vec{S}_1 \cdot \vec{a}_2 \right)^2 - 2 \hat{n} \cdot \vec{S}_1 \hat{n} \cdot \vec{v}_2 \vec{S}_1 \cdot \vec{a}_2 + 2 \left( \hat{n} \cdot \vec{S}_1 \right)^2 \vec{a}_2 \cdot \vec{a}_2 - 2 \hat{n} \cdot \vec{S}_1 \hat{n} \cdot \vec{v}_2 \vec{S}_1 \cdot \vec{a}_2 + \\ & \left. \left. 2 \vec{S}_1 \cdot \vec{v}_2 \vec{S}_1 \cdot \vec{a}_2 - 4 \vec{a}_2 \cdot \vec{a}_2 \vec{S}_1 \cdot \vec{S}_1 + 2 \vec{S}_1 \cdot \vec{a}_2 \vec{S}_1 \cdot \vec{v}_2 + 4 \hat{n} \cdot \vec{S}_1 \hat{n} \cdot \vec{S}_1 \vec{v}_2 \cdot \vec{a}_2 - 8 \vec{S}_1 \cdot \vec{S}_1 \vec{v}_2 \cdot \vec{a}_2 \right) + \frac{1}{\rho^3} \right. \\ & \left( 8 \vec{S}_1 \cdot \vec{S}_1 \left( \hat{n} \cdot \vec{v}_2 \right)^3 - 4 \hat{n} \cdot \vec{S}_1 \vec{S}_1 \cdot \vec{v}_2 \left( \hat{n} \cdot \vec{v}_2 \right)^2 - 8 \hat{n} \cdot \vec{S}_1 \vec{S}_1 \cdot \vec{a}_2 \left( \hat{n} \cdot \vec{v}_2 \right)^2 + 16 \hat{n} \cdot \vec{a}_2 \vec{S}_1 \cdot \vec{S}_1 \left( \hat{n} \cdot \vec{v}_2 \right)^2 - \right. \\ & 4 \hat{n} \cdot \vec{S}_1 \vec{S}_1 \cdot \vec{v}_2 \left( \hat{n} \cdot \vec{v}_2 \right)^2 + 8 \hat{n} \cdot \vec{S}_1 \hat{n} \cdot \vec{v}_1 \vec{S}_1 \cdot \vec{a}_2 \hat{n} \cdot \vec{v}_2 - 16 \hat{n} \cdot \vec{a}_2 \hat{n} \cdot \vec{v}_1 \vec{S}_1 \cdot \vec{S}_1 \hat{n} \cdot \vec{v}_2 - 2 \vec{S}_1 \cdot \vec{a}_2 \vec{S}_1 \cdot \vec{v}_1 \hat{n} \cdot \vec{v}_2 - \\ & 8 \hat{n} \cdot \vec{a}_2 \hat{n} \cdot \vec{S}_1 \vec{S}_1 \cdot \vec{v}_2 \hat{n} \cdot \vec{v}_2 + 4 \vec{S}_1 \cdot \vec{v}_2 \vec{S}_1 \cdot \vec{v}_2 \hat{n} \cdot \vec{v}_2 + 8 \vec{S}_1 \cdot \vec{a}_2 \vec{S}_1 \cdot \vec{v}_2 \hat{n} \cdot \vec{v}_2 + 4 \vec{S}_1 \cdot \vec{S}_1 \vec{v}_1 \cdot \vec{a}_2 \hat{n} \cdot \vec{v}_2 + \\ & 8 \left( \hat{n} \cdot \vec{S}_1 \right)^2 \vec{v}_2 \cdot \vec{a}_2 \hat{n} \cdot \vec{v}_2 - 16 \vec{S}_1 \cdot \vec{S}_1 \vec{v}_2 \cdot \vec{a}_2 \hat{n} \cdot \vec{v}_2 + 4 \hat{n} \cdot \vec{S}_1 \hat{n} \cdot \vec{S}_1 \vec{v}_2 \cdot \vec{v}_2 \hat{n} \cdot \vec{v}_2 - 8 \vec{S}_1 \cdot \vec{S}_1 \vec{v}_2 \cdot \vec{v}_2 \hat{n} \cdot \vec{v}_2 + \\ & 8 \hat{n} \cdot \vec{a}_2 \hat{n} \cdot \vec{S}_1 \hat{n} \cdot \vec{v}_1 \vec{S}_1 \cdot \vec{v}_2 - 4 \hat{n} \cdot \vec{v}_1 \vec{S}_1 \cdot \vec{a}_2 \vec{S}_1 \cdot \vec{v}_2 - 2 \hat{n} \cdot \vec{a}_2 \vec{S}_1 \cdot \vec{v}_1 \vec{S}_1 \cdot \vec{v}_2 - 2 \hat{n} \cdot \vec{S}_1 \vec{S}_1 \cdot \vec{v}_2 \vec{v}_1 \cdot \vec{a}_2 - 2 \hat{n} \cdot \vec{S}_1 \vec{S}_1 \cdot \vec{v}_2 \vec{v}_1 \cdot \vec{v}_2 + \\ & \left. \left. \vec{v}_1 \cdot \vec{v}_2 + 4 \hat{n} \cdot \vec{a}_2 \vec{S}_1 \cdot \vec{S}_1 \vec{v}_1 \cdot \vec{v}_2 - 8 \left( \hat{n} \cdot \vec{S}_1 \right)^2 \hat{n} \cdot \vec{v}_1 \vec{v}_2 \cdot \vec{a}_2 + 8 \hat{n} \cdot \vec{v}_1 \vec{S}_1 \cdot \vec{S}_1 \vec{v}_2 \cdot \vec{a}_2 + 4 \hat{n} \cdot \vec{S}_1 \vec{S}_1 \cdot \vec{v}_1 \vec{v}_2 \cdot \vec{a}_2 \right) + \right. \\ & \left. \frac{1}{\rho^4} \left( 12 \vec{S}_1 \cdot \vec{S}_1 \left( \hat{n} \cdot \vec{v}_2 \right)^4 - 24 \hat{n} \cdot \vec{v}_1 \vec{S}_1 \cdot \vec{S}_1 \left( \hat{n} \cdot \vec{v}_2 \right)^3 - 12 \hat{n} \cdot \vec{S}_1 \vec{S}_1 \cdot \vec{v}_2 \left( \hat{n} \cdot \vec{v}_2 \right)^3 + 6 \left( \vec{S}_1 \cdot \vec{v}_2 \right)^2 \left( \hat{n} \cdot \vec{v}_2 \right)^2 + \right. \\ & 24 \hat{n} \cdot \vec{S}_1 \hat{n} \cdot \vec{v}_1 \vec{S}_1 \cdot \vec{v}_2 \left( \hat{n} \cdot \vec{v}_2 \right)^2 - 4 \vec{S}_1 \cdot \vec{v}_1 \vec{S}_1 \cdot \vec{v}_2 \left( \hat{n} \cdot \vec{v}_2 \right)^2 + 12 \vec{S}_1 \cdot \vec{S}_1 \vec{v}_1 \cdot \vec{v}_2 \left( \hat{n} \cdot \vec{v}_2 \right)^2 + \\ & 6 \left( \hat{n} \cdot \vec{S}_1 \right)^2 \vec{v}_2 \cdot \vec{v}_2 \left( \hat{n} \cdot \vec{v}_2 \right)^2 - 12 \vec{S}_1 \cdot \vec{S}_1 \vec{v}_2 \cdot \vec{v}_2 \left( \hat{n} \cdot \vec{v}_2 \right)^2 - 8 \hat{n} \cdot \vec{v}_1 \left( \vec{S}_1 \cdot \vec{v}_2 \right)^2 \hat{n} \cdot \vec{v}_2 - \\ & \left. \left. 8 \hat{n} \cdot \vec{S}_1 \vec{S}_1 \cdot \vec{v}_2 \vec{v}_1 \cdot \vec{v}_2 \hat{n} \cdot \vec{v}_2 - 12 \left( \hat{n} \cdot \vec{S}_1 \right)^2 \hat{n} \cdot \vec{v}_1 \vec{v}_2 \cdot \vec{v}_2 \hat{n} \cdot \vec{v}_2 + 16 \hat{n} \cdot \vec{v}_1 \vec{S}_1 \cdot \vec{S}_1 \vec{v}_2 \cdot \vec{v}_2 \hat{n} \cdot \vec{v}_2 + \right. \right. \end{aligned}$$

$$4 \hat{n} \cdot \vec{S}_1 \vec{S}_1 \cdot \vec{v}_1 \vec{v}_2 \cdot \vec{v}_2 \hat{n} \cdot \vec{v}_2 + 2 \left( \vec{S}_1 \cdot \vec{v}_2 \right)^2 \vec{v}_1 \cdot \vec{v}_2 + 2 \left( \hat{n} \cdot \vec{S}_1 \right)^2 \vec{v}_1 \cdot \vec{v}_2 \vec{v}_2 \cdot \vec{v}_2 - 4 \vec{S}_1 \cdot \vec{S}_1 \vec{v}_1 \cdot \vec{v}_2 \vec{v}_2 \cdot \vec{v}_2 \right) \left. m_2^2 C_{ES^2 1} \right\}$$

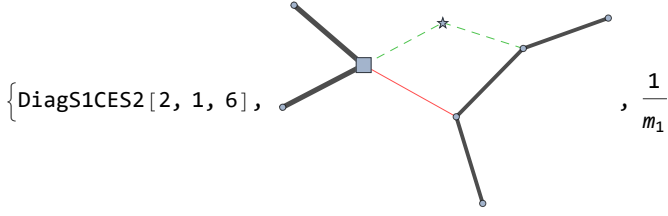

$$\begin{aligned} G^2 \left( \frac{1}{r^4} \left( 48 \vec{S}_1 \cdot \vec{S}_1 (\hat{n} \cdot \vec{v}_2)^4 - 132 \hat{n} \cdot \vec{v}_1 \vec{S}_1 \cdot \vec{S}_1 (\hat{n} \cdot \vec{v}_2)^3 + 3 \hat{n} \cdot \vec{S}_1 \vec{S}_1 \cdot \vec{v}_1 (\hat{n} \cdot \vec{v}_2)^3 - 54 \hat{n} \cdot \vec{S}_1 \vec{S}_1 \cdot \vec{v}_2 (\hat{n} \cdot \vec{v}_2)^3 + \right. \right. \\ \left( \vec{S}_1 \cdot \vec{v}_1 \right)^2 (\hat{n} \cdot \vec{v}_2)^2 + 25 \left( \vec{S}_1 \cdot \vec{v}_2 \right)^2 (\hat{n} \cdot \vec{v}_2)^2 + 84 (\hat{n} \cdot \vec{v}_1)^2 \vec{S}_1 \cdot \vec{S}_1 (\hat{n} \cdot \vec{v}_2)^2 - 6 \hat{n} \cdot \vec{S}_1 \hat{n} \cdot \vec{v}_1 \vec{S}_1 \cdot \vec{v}_1 (\hat{n} \cdot \vec{v}_2)^2 + \\ 147 \hat{n} \cdot \vec{S}_1 \hat{n} \cdot \vec{v}_1 \vec{S}_1 \cdot \vec{v}_2 (\hat{n} \cdot \vec{v}_2)^2 - 25 \vec{S}_1 \cdot \vec{v}_1 \vec{S}_1 \cdot \vec{v}_2 (\hat{n} \cdot \vec{v}_2)^2 - 14 \vec{S}_1 \cdot \vec{S}_1 \vec{v}_1 \cdot \vec{v}_1 (\hat{n} \cdot \vec{v}_2)^2 - \\ 42 (\hat{n} \cdot \vec{S}_1)^2 \vec{v}_1 \cdot \vec{v}_2 (\hat{n} \cdot \vec{v}_2)^2 + 70 \vec{S}_1 \cdot \vec{S}_1 \vec{v}_1 \cdot \vec{v}_2 (\hat{n} \cdot \vec{v}_2)^2 - 39 \vec{S}_1 \cdot \vec{S}_1 \vec{v}_2 \cdot \vec{v}_2 (\hat{n} \cdot \vec{v}_2)^2 - \\ 45 \hat{n} \cdot \vec{v}_1 \left( \vec{S}_1 \cdot \vec{v}_2 \right)^2 \hat{n} \cdot \vec{v}_2 - 90 \hat{n} \cdot \vec{S}_1 (\hat{n} \cdot \vec{v}_1)^2 \vec{S}_1 \cdot \vec{v}_2 \hat{n} \cdot \vec{v}_2 + 31 \hat{n} \cdot \vec{v}_1 \vec{S}_1 \cdot \vec{v}_1 \vec{S}_1 \cdot \vec{v}_2 \hat{n} \cdot \vec{v}_2 + \\ 15 \hat{n} \cdot \vec{S}_1 \vec{S}_1 \cdot \vec{v}_2 \vec{v}_1 \cdot \vec{v}_1 \hat{n} \cdot \vec{v}_2 + 108 (\hat{n} \cdot \vec{S}_1)^2 \hat{n} \cdot \vec{v}_1 \vec{v}_1 \cdot \vec{v}_2 \hat{n} \cdot \vec{v}_2 - 64 \hat{n} \cdot \vec{v}_1 \vec{S}_1 \cdot \vec{S}_1 \vec{v}_1 \cdot \vec{v}_2 \hat{n} \cdot \vec{v}_2 - \\ 34 \hat{n} \cdot \vec{S}_1 \vec{S}_1 \cdot \vec{v}_1 \vec{v}_1 \cdot \vec{v}_2 \hat{n} \cdot \vec{v}_2 - 25 \hat{n} \cdot \vec{S}_1 \vec{S}_1 \cdot \vec{v}_2 \vec{v}_1 \cdot \vec{v}_2 \hat{n} \cdot \vec{v}_2 + 64 \hat{n} \cdot \vec{v}_1 \vec{S}_1 \cdot \vec{S}_1 \vec{v}_2 \cdot \vec{v}_2 \hat{n} \cdot \vec{v}_2 - \\ \hat{n} \cdot \vec{S}_1 \vec{S}_1 \cdot \vec{v}_1 \vec{v}_2 \cdot \vec{v}_2 \hat{n} \cdot \vec{v}_2 + 22 \hat{n} \cdot \vec{S}_1 \vec{S}_1 \cdot \vec{v}_2 \vec{v}_2 \cdot \vec{v}_2 \hat{n} \cdot \vec{v}_2 + 12 (\hat{n} \cdot \vec{v}_1)^2 \left( \vec{S}_1 \cdot \vec{v}_2 \right)^2 - 18 (\hat{n} \cdot \vec{S}_1)^2 (\vec{v}_1 \cdot \vec{v}_2)^2 + \\ 9 \vec{S}_1 \cdot \vec{S}_1 (\vec{v}_1 \cdot \vec{v}_2)^2 + 3 \vec{S}_1 \cdot \vec{S}_1 (\vec{v}_2 \cdot \vec{v}_2)^2 - 3 \left( \vec{S}_1 \cdot \vec{v}_2 \right)^2 \vec{v}_1 \cdot \vec{v}_1 + 9 \left( \vec{S}_1 \cdot \vec{v}_2 \right)^2 \vec{v}_1 \cdot \vec{v}_2 + \\ 3 \hat{n} \cdot \vec{S}_1 \hat{n} \cdot \vec{v}_1 \vec{S}_1 \cdot \vec{v}_2 \vec{v}_1 \cdot \vec{v}_2 - \vec{S}_1 \cdot \vec{v}_1 \vec{S}_1 \cdot \vec{v}_2 \vec{v}_1 \cdot \vec{v}_2 - 5 \left( \vec{S}_1 \cdot \vec{v}_2 \right)^2 \vec{v}_2 \cdot \vec{v}_2 - 12 (\hat{n} \cdot \vec{v}_1)^2 \vec{S}_1 \cdot \vec{S}_1 \vec{v}_2 \cdot \vec{v}_2 - \\ 28 \hat{n} \cdot \vec{S}_1 \hat{n} \cdot \vec{v}_1 \vec{S}_1 \cdot \vec{v}_2 \vec{v}_2 \cdot \vec{v}_2 + 7 \vec{S}_1 \cdot \vec{v}_1 \vec{S}_1 \cdot \vec{v}_2 \vec{v}_2 \cdot \vec{v}_2 + 3 \vec{S}_1 \cdot \vec{S}_1 \vec{v}_1 \cdot \vec{v}_1 \vec{v}_2 \cdot \vec{v}_2 - 14 \vec{S}_1 \cdot \vec{S}_1 \vec{v}_1 \cdot \vec{v}_2 \vec{v}_2 \cdot \vec{v}_2 \Big) + \\ \frac{\hat{n} \cdot \vec{S}_1 \vec{S}_1 \cdot \vec{a}_2 + \hat{n} \cdot \vec{S}_1 \vec{S}_1 \cdot \vec{a}_2 - 2 \hat{n} \cdot \vec{a}_2 \vec{S}_1 \cdot \vec{S}_1 + 2 \hat{n} \cdot \vec{a}_2 \vec{S}_1^2}{r} + \frac{1}{r^2} \\ \left( -5 \vec{S}_1 \cdot \vec{S}_1 (\hat{n} \cdot \vec{a}_2)^2 + \hat{n} \cdot \vec{S}_1 \vec{S}_1 \cdot \vec{v}_1 \hat{n} \cdot \vec{a}_2 - 7 \hat{n} \cdot \vec{S}_1 \vec{S}_1 \cdot \vec{v}_2 \hat{n} \cdot \vec{a}_2 - 20 \hat{n} \cdot \vec{v}_1 \vec{S}_1 \cdot \vec{S}_1 \hat{n} \cdot \vec{a}_2 + 32 \hat{n} \cdot \vec{v}_2 \vec{S}_1 \cdot \vec{S}_1 \hat{n} \cdot \vec{a}_2 + \right. \\ \hat{n} \cdot \vec{S}_1 \vec{S}_1 \cdot \vec{a}_1 \hat{n} \cdot \vec{a}_2 + 5 \hat{n} \cdot \vec{S}_1 \vec{S}_1 \cdot \vec{a}_2 \hat{n} \cdot \vec{a}_2 - 8 \hat{n} \cdot \vec{a}_1 \vec{S}_1 \cdot \vec{S}_1 \hat{n} \cdot \vec{a}_2 + \hat{n} \cdot \vec{S}_1 \vec{S}_1 \cdot \vec{v}_1 \hat{n} \cdot \vec{a}_2 - 7 \hat{n} \cdot \vec{S}_1 \vec{S}_1 \cdot \vec{v}_2 \hat{n} \cdot \vec{a}_2 + \\ 2 \hat{n} \cdot \vec{v}_1 \vec{S}_1^2 \hat{n} \cdot \vec{a}_2 - 6 \hat{n} \cdot \vec{v}_2 \vec{S}_1^2 \hat{n} \cdot \vec{a}_2 - 2 \left( \vec{S}_1 \cdot \vec{a}_2 \right)^2 + 9 \hat{n} \cdot \vec{S}_1 \hat{n} \cdot \vec{v}_1 \vec{S}_1 \cdot \vec{a}_2 - 9 \hat{n} \cdot \vec{S}_1 \hat{n} \cdot \vec{v}_2 \vec{S}_1 \cdot \vec{a}_2 - 6 (\hat{n} \cdot \vec{S}_1)^2 \vec{a}_1 \cdot \vec{a}_2 - \\ 2 \hat{n} \cdot \vec{S}_1 \hat{n} \cdot \vec{v}_1 \vec{S}_1 \cdot \vec{a}_2 + 9 \hat{n} \cdot \vec{S}_1 \hat{n} \cdot \vec{v}_2 \vec{S}_1 \cdot \vec{a}_2 + 9 \hat{n} \cdot \vec{a}_1 \hat{n} \cdot \vec{S}_1 \vec{S}_1 \cdot \vec{a}_2 + 9 \hat{n} \cdot \vec{S}_1 \hat{n} \cdot \vec{v}_1 \vec{S}_1 \cdot \vec{a}_2 - 9 \hat{n} \cdot \vec{S}_1 \hat{n} \cdot \vec{v}_2 \vec{S}_1 \cdot \vec{a}_2 - \\ 4 \vec{S}_1 \cdot \vec{v}_1 \vec{S}_1 \cdot \vec{a}_2 + 7 \vec{S}_1 \cdot \vec{v}_2 \vec{S}_1 \cdot \vec{a}_2 - 4 \vec{S}_1 \cdot \vec{a}_1 \vec{S}_1 \cdot \vec{a}_2 - 2 \hat{n} \cdot \vec{a}_2 \hat{n} \cdot \vec{v}_1 \vec{S}_1 \cdot \vec{S}_1 - 3 \hat{n} \cdot \vec{a}_2 \hat{n} \cdot \vec{v}_2 \vec{S}_1 \cdot \vec{S}_1 + \\ 4 \vec{a}_1 \cdot \vec{a}_2 \vec{S}_1 \cdot \vec{S}_1 + 2 \vec{a}_2 \cdot \vec{a}_2 \vec{S}_1 \cdot \vec{S}_1 - 4 \vec{S}_1 \cdot \vec{a}_2 \vec{S}_1 \cdot \vec{v}_1 + \vec{S}_1 \cdot \vec{a}_2 \vec{S}_1 \cdot \vec{v}_1 + 7 \vec{S}_1 \cdot \vec{a}_2 \vec{S}_1 \cdot \vec{v}_2 - 4 \vec{S}_1 \cdot \vec{a}_2 \vec{S}_1 \cdot \vec{v}_2 + \\ \vec{S}_1 \cdot \vec{S}_1 \vec{v}_1 \cdot \vec{a}_2 - 12 \hat{n} \cdot \vec{S}_1 \hat{n} \cdot \vec{S}_1 \vec{v}_1 \cdot \vec{a}_2 + 12 \vec{S}_1 \cdot \vec{S}_1 \vec{v}_1 \cdot \vec{a}_2 + 2 \vec{S}_1 \cdot \vec{S}_1 \vec{v}_2 \cdot \vec{a}_2 - 14 \vec{S}_1 \cdot \vec{S}_1 \vec{v}_2 \cdot \vec{a}_2 - 2 \vec{v}_1 \cdot \vec{a}_2 \vec{S}_1^2 \Big) + \\ \frac{1}{r^3} \left( 40 \vec{S}_1 \cdot \vec{S}_1 (\hat{n} \cdot \vec{v}_2)^3 - 2 \vec{S}_1^2 (\hat{n} \cdot \vec{v}_2)^3 + \hat{n} \cdot \vec{S}_1 \vec{S}_1 \cdot \vec{v}_1 (\hat{n} \cdot \vec{v}_2)^2 - 20 \hat{n} \cdot \vec{S}_1 \vec{S}_1 \cdot \vec{v}_2 (\hat{n} \cdot \vec{v}_2)^2 - \right. \\ 32 \hat{n} \cdot \vec{v}_1 \vec{S}_1 \cdot \vec{S}_1 (\hat{n} \cdot \vec{v}_2)^2 + \hat{n} \cdot \vec{S}_1 \vec{S}_1 \cdot \vec{a}_1 (\hat{n} \cdot \vec{v}_2)^2 - 3 \hat{n} \cdot \vec{S}_1 \vec{S}_1 \cdot \vec{a}_2 (\hat{n} \cdot \vec{v}_2)^2 - 14 \hat{n} \cdot \vec{a}_1 \vec{S}_1 \cdot \vec{S}_1 (\hat{n} \cdot \vec{v}_2)^2 + \\ 7 \hat{n} \cdot \vec{a}_2 \vec{S}_1 \cdot \vec{S}_1 (\hat{n} \cdot \vec{v}_2)^2 + \hat{n} \cdot \vec{S}_1 \vec{S}_1 \cdot \vec{v}_1 (\hat{n} \cdot \vec{v}_2)^2 - 20 \hat{n} \cdot \vec{S}_1 \vec{S}_1 \cdot \vec{v}_2 (\hat{n} \cdot \vec{v}_2)^2 + 2 \hat{n} \cdot \vec{v}_1 \vec{S}_1^2 (\hat{n} \cdot \vec{v}_2)^2 + \\ 15 \hat{n} \cdot \vec{S}_1 \hat{n} \cdot \vec{v}_1 \vec{S}_1 \cdot \vec{v}_2 \hat{n} \cdot \vec{v}_2 - 18 (\hat{n} \cdot \vec{S}_1)^2 \vec{a}_1 \cdot \vec{v}_2 \hat{n} \cdot \vec{v}_2 + 57 \hat{n} \cdot \vec{S}_1 \hat{n} \cdot \vec{v}_1 \vec{S}_1 \cdot \vec{a}_2 \hat{n} \cdot \vec{v}_2 - 58 \hat{n} \cdot \vec{a}_2 \hat{n} \cdot \vec{v}_1 \vec{S}_1 \cdot \vec{S}_1 \hat{n} \cdot \vec{v}_2 + \\ 9 \vec{a}_1 \cdot \vec{v}_2 \vec{S}_1 \cdot \vec{S}_1 \hat{n} \cdot \vec{v}_2 + 3 \hat{n} \cdot \vec{a}_2 \hat{n} \cdot \vec{S}_1 \vec{S}_1 \cdot \vec{v}_1 \hat{n} \cdot \vec{v}_2 - 4 \vec{S}_1 \cdot \vec{v}_2 \vec{S}_1 \cdot \vec{v}_1 \hat{n} \cdot \vec{v}_2 - 14 \vec{S}_1 \cdot \vec{a}_2 \vec{S}_1 \cdot \vec{v}_1 \hat{n} \cdot \vec{v}_2 + \\ 15 \hat{n} \cdot \vec{a}_1 \hat{n} \cdot \vec{S}_1 \vec{S}_1 \cdot \vec{v}_2 \hat{n} \cdot \vec{v}_2 - 22 \hat{n} \cdot \vec{a}_2 \hat{n} \cdot \vec{S}_1 \vec{S}_1 \cdot \vec{v}_2 \hat{n} \cdot \vec{v}_2 + 15 \hat{n} \cdot \vec{S}_1 \hat{n} \cdot \vec{v}_1 \vec{S}_1 \cdot \vec{v}_2 \hat{n} \cdot \vec{v}_2 - 4 \vec{S}_1 \cdot \vec{v}_1 \vec{S}_1 \cdot \vec{v}_2 \hat{n} \cdot \vec{v}_2 + \\ 18 \vec{S}_1 \cdot \vec{v}_2 \vec{S}_1 \cdot \vec{v}_2 \hat{n} \cdot \vec{v}_2 - 4 \vec{S}_1 \cdot \vec{a}_1 \vec{S}_1 \cdot \vec{v}_2 \hat{n} \cdot \vec{v}_2 + 7 \vec{S}_1 \cdot \vec{a}_2 \vec{S}_1 \cdot \vec{v}_2 \hat{n} \cdot \vec{v}_2 - 6 (\hat{n} \cdot \vec{S}_1)^2 \vec{v}_1 \cdot \vec{a}_2 \hat{n} \cdot \vec{v}_2 + \end{aligned}$$

$$\begin{aligned}
& 17 \vec{S}_1 \cdot \vec{S}_1 \vec{v}_1 \cdot \vec{a}_2 \hat{n} \cdot \vec{v}_2 - 36 \hat{n} \cdot \vec{S}_1 \hat{n} \cdot \vec{S}_1 \vec{v}_1 \cdot \vec{v}_2 \hat{n} \cdot \vec{v}_2 + 22 \vec{S}_1 \cdot \vec{S}_1 \vec{v}_1 \cdot \vec{v}_2 \hat{n} \cdot \vec{v}_2 - 3 \vec{S}_1 \cdot \vec{S}_1 \vec{v}_2 \cdot \vec{a}_2 \hat{n} \cdot \vec{v}_2 - \\
& 32 \vec{S}_1 \cdot \vec{S}_1 \vec{v}_2 \cdot \vec{v}_2 \hat{n} \cdot \vec{v}_2 - 2 \vec{v}_1 \cdot \vec{v}_2 \vec{S}_1^1 \hat{n} \cdot \vec{v}_2 + 2 \vec{v}_2 \cdot \vec{v}_2 \vec{S}_1^1 \hat{n} \cdot \vec{v}_2 + \hat{n} \cdot \vec{a}_2 \left( \vec{S}_1 \cdot \vec{v}_1 \right)^2 - 3 \hat{n} \cdot \vec{a}_1 \left( \vec{S}_1 \cdot \vec{v}_2 \right)^2 + \\
& 5 \hat{n} \cdot \vec{a}_2 \left( \vec{S}_1 \cdot \vec{v}_2 \right)^2 - 36 \hat{n} \cdot \vec{S}_1 \left( \hat{n} \cdot \vec{v}_1 \right)^2 \vec{S}_1 \cdot \vec{a}_2 + 32 \hat{n} \cdot \vec{a}_2 \left( \hat{n} \cdot \vec{v}_1 \right)^2 \vec{S}_1 \cdot \vec{S}_1 - 4 \hat{n} \cdot \vec{a}_2 \hat{n} \cdot \vec{S}_1 \hat{n} \cdot \vec{v}_1 \vec{S}_1 \cdot \vec{v}_1 + \\
& 17 \hat{n} \cdot \vec{v}_1 \vec{S}_1 \cdot \vec{a}_2 \vec{S}_1 \cdot \vec{v}_1 + 28 \hat{n} \cdot \vec{a}_2 \hat{n} \cdot \vec{S}_1 \hat{n} \cdot \vec{v}_1 \vec{S}_1 \cdot \vec{v}_2 - 6 \hat{n} \cdot \vec{v}_1 \vec{S}_1 \cdot \vec{v}_2 \vec{S}_1 \cdot \vec{v}_2 + 3 \hat{n} \cdot \vec{S}_1 \vec{a}_1 \cdot \vec{v}_2 \vec{S}_1 \cdot \vec{v}_2 - \\
& 20 \hat{n} \cdot \vec{v}_1 \vec{S}_1 \cdot \vec{a}_2 \vec{S}_1 \cdot \vec{v}_2 - 7 \hat{n} \cdot \vec{a}_2 \vec{S}_1 \cdot \vec{v}_1 \vec{S}_1 \cdot \vec{v}_2 + 24 \left( \hat{n} \cdot \vec{S}_1 \right)^2 \hat{n} \cdot \vec{v}_1 \vec{v}_1 \cdot \vec{a}_2 - 16 \hat{n} \cdot \vec{v}_1 \vec{S}_1 \cdot \vec{S}_1 \vec{v}_1 \cdot \vec{a}_2 - \\
& 11 \hat{n} \cdot \vec{S}_1 \vec{S}_1 \cdot \vec{v}_1 \vec{v}_1 \cdot \vec{a}_2 - 7 \hat{n} \cdot \vec{S}_1 \vec{S}_1 \cdot \vec{v}_2 \vec{v}_1 \cdot \vec{a}_2 + 9 \hat{n} \cdot \vec{S}_1 \vec{S}_1 \cdot \vec{a}_2 \vec{v}_1 \cdot \vec{v}_1 - 8 \hat{n} \cdot \vec{a}_2 \vec{S}_1 \cdot \vec{S}_1 \vec{v}_1 \cdot \vec{v}_1 + \\
& 3 \hat{n} \cdot \vec{S}_1 \vec{S}_1 \cdot \vec{v}_2 \vec{v}_1 \cdot \vec{v}_2 - 9 \hat{n} \cdot \vec{S}_1 \vec{S}_1 \cdot \vec{a}_2 \vec{v}_1 \cdot \vec{v}_2 + 10 \hat{n} \cdot \vec{a}_2 \vec{S}_1 \cdot \vec{S}_1 \vec{v}_1 \cdot \vec{v}_2 + 3 \hat{n} \cdot \vec{S}_1 \vec{S}_1 \cdot \vec{v}_2 \vec{v}_1 \cdot \vec{v}_2 + \\
& 19 \hat{n} \cdot \vec{v}_1 \vec{S}_1 \cdot \vec{S}_1 \vec{v}_2 \cdot \vec{a}_2 - \hat{n} \cdot \vec{S}_1 \vec{S}_1 \cdot \vec{v}_1 \vec{v}_2 \cdot \vec{a}_2 + 7 \hat{n} \cdot \vec{S}_1 \vec{S}_1 \cdot \vec{v}_2 \vec{v}_2 \cdot \vec{v}_2 + 6 \hat{n} \cdot \vec{v}_1 \vec{S}_1 \cdot \vec{S}_1 \vec{v}_2 \cdot \vec{v}_2 - \\
& 5 \hat{n} \cdot \vec{S}_1 \vec{S}_1 \cdot \vec{a}_2 \vec{v}_2 \cdot \vec{v}_2 + 3 \hat{n} \cdot \vec{a}_1 \vec{S}_1 \cdot \vec{S}_1 \vec{v}_2 \cdot \vec{v}_2 + 2 \hat{n} \cdot \vec{a}_2 \vec{S}_1 \cdot \vec{S}_1 \vec{v}_2 \cdot \vec{v}_2 + 7 \hat{n} \cdot \vec{S}_1 \vec{S}_1 \cdot \vec{v}_2 \vec{v}_2 \cdot \vec{v}_2 \Bigg) m_2^2 C_{ES^2_1} \Bigg\}
\end{aligned}$$

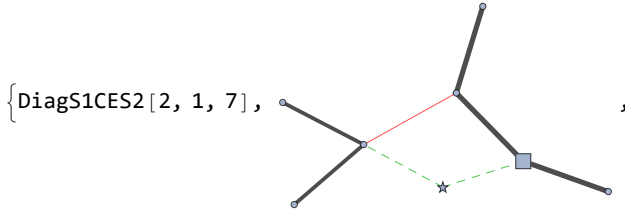

$$\begin{aligned}
& G^2 \left( \frac{-2 \hat{n} \cdot \vec{a}_2 \vec{S}_1 \cdot \vec{S}_1 + 2 \hat{n} \cdot \vec{S}_1 \vec{S}_1 \cdot \vec{a}_2 + \hat{n} \cdot \vec{S}_1 \vec{S}_1^2 \cdot \vec{a}_2 - 2 \hat{n} \cdot \vec{a}_2 \vec{S}_1 \cdot \vec{S}_1 + \hat{n} \cdot \vec{S}_1 \vec{S}_1 \cdot \vec{a}_2}{r} + \frac{1}{r^4} \right. \\
& \left( -3 \left( \vec{v}_1 \cdot \vec{v}_2 \right)^2 \left( \hat{n} \cdot \vec{S}_1 \right)^2 - 3 \left( \hat{n} \cdot \vec{v}_1 \right)^2 \vec{v}_1 \cdot \vec{v}_2 \left( \hat{n} \cdot \vec{S}_1 \right)^2 + 18 \hat{n} \cdot \vec{v}_1 \hat{n} \cdot \vec{v}_2 \vec{v}_1 \cdot \vec{v}_2 \left( \hat{n} \cdot \vec{S}_1 \right)^2 + \right. \\
& 2 \hat{n} \cdot \vec{v}_1 \vec{S}_1 \cdot \vec{v}_1 \vec{v}_1 \cdot \vec{v}_2 \hat{n} \cdot \vec{S}_1 - 8 \hat{n} \cdot \vec{v}_2 \vec{S}_1 \cdot \vec{v}_1 \vec{v}_1 \cdot \vec{v}_2 \hat{n} \cdot \vec{S}_1 - 6 \hat{n} \cdot \vec{v}_1 \vec{S}_1 \cdot \vec{v}_2 \vec{v}_1 \cdot \vec{v}_2 \hat{n} \cdot \vec{S}_1 - \\
& \left. \vec{S}_1 \cdot \vec{S}_1 \left( \vec{v}_1 \cdot \vec{v}_2 \right)^2 - \left( \hat{n} \cdot \vec{v}_1 \right)^2 \vec{S}_1 \cdot \vec{S}_1 \vec{v}_1 \cdot \vec{v}_2 + 4 \hat{n} \cdot \vec{v}_1 \hat{n} \cdot \vec{v}_2 \vec{S}_1 \cdot \vec{S}_1 \vec{v}_1 \cdot \vec{v}_2 + 2 \vec{S}_1 \cdot \vec{v}_1 \vec{S}_1 \cdot \vec{v}_2 \vec{v}_1 \cdot \vec{v}_2 \right) + \frac{1}{r^3} \\
& \left( \hat{n} \cdot \vec{v}_1 \vec{a}_1 \cdot \vec{v}_2 \left( \hat{n} \cdot \vec{S}_1 \right)^2 - 4 \hat{n} \cdot \vec{v}_2 \vec{a}_1 \cdot \vec{v}_2 \left( \hat{n} \cdot \vec{S}_1 \right)^2 + 3 \hat{n} \cdot \vec{v}_1 \vec{v}_1 \cdot \vec{a}_2 \left( \hat{n} \cdot \vec{S}_1 \right)^2 + \left( \hat{n} \cdot \vec{v}_1 \right)^2 \vec{S}_1 \cdot \vec{v}_2 \hat{n} \cdot \vec{S}_1 - \right. \\
& 4 \hat{n} \cdot \vec{v}_1 \hat{n} \cdot \vec{v}_2 \vec{S}_1 \cdot \vec{v}_2 \hat{n} \cdot \vec{S}_1 + 2 \vec{a}_1 \cdot \vec{v}_2 \vec{S}_1 \cdot \vec{v}_2 \hat{n} \cdot \vec{S}_1 - 2 \vec{S}_1 \cdot \vec{v}_1 \vec{v}_1 \cdot \vec{a}_2 \hat{n} \cdot \vec{S}_1 + 2 \hat{n} \cdot \vec{S}_1 \hat{n} \cdot \vec{v}_1 \vec{v}_1 \cdot \vec{v}_2 \hat{n} \cdot \vec{S}_1 - \\
& 8 \hat{n} \cdot \vec{S}_1 \hat{n} \cdot \vec{v}_2 \vec{v}_1 \cdot \vec{v}_2 \hat{n} \cdot \vec{S}_1 + 3 \vec{S}_1 \cdot \vec{v}_2 \vec{v}_1 \cdot \vec{v}_2 \hat{n} \cdot \vec{S}_1 + 8 \hat{n} \cdot \vec{v}_1 \left( \hat{n} \cdot \vec{v}_2 \right)^2 \vec{S}_1 \cdot \vec{S}_1 - 2 \left( \hat{n} \cdot \vec{v}_1 \right)^2 \hat{n} \cdot \vec{v}_2 \vec{S}_1 \cdot \vec{S}_1 + \\
& \hat{n} \cdot \vec{v}_1 \vec{a}_1 \cdot \vec{v}_2 \vec{S}_1 \cdot \vec{S}_1 - 2 \hat{n} \cdot \vec{v}_2 \vec{a}_1 \cdot \vec{v}_2 \vec{S}_1 \cdot \vec{S}_1 - \hat{n} \cdot \vec{v}_1 \vec{S}_1 \cdot \vec{v}_2 \vec{S}_1 \cdot \vec{v}_1 + 2 \hat{n} \cdot \vec{v}_2 \vec{S}_1 \cdot \vec{v}_2 \vec{S}_1 \cdot \vec{v}_1 + \hat{n} \cdot \vec{S}_1 \left( \hat{n} \cdot \vec{v}_1 \right)^2 \vec{S}_1 \cdot \vec{v}_2 - \\
& 4 \hat{n} \cdot \vec{S}_1 \hat{n} \cdot \vec{v}_1 \hat{n} \cdot \vec{v}_2 \vec{S}_1 \cdot \vec{v}_2 - \hat{n} \cdot \vec{v}_1 \vec{S}_1 \cdot \vec{v}_1 \vec{S}_1 \cdot \vec{v}_2 + 2 \hat{n} \cdot \vec{v}_2 \vec{S}_1 \cdot \vec{v}_1 \vec{S}_1 \cdot \vec{v}_2 + 2 \hat{n} \cdot \vec{v}_1 \vec{S}_1 \cdot \vec{v}_2 \vec{S}_1 \cdot \vec{v}_2 + \hat{n} \cdot \vec{v}_1 \vec{S}_1 \cdot \vec{S}_1 \\
& \left. \vec{v}_1 \cdot \vec{a}_2 + 4 \hat{n} \cdot \vec{v}_1 \vec{S}_1 \cdot \vec{S}_1 \vec{v}_1 \cdot \vec{v}_2 - 10 \hat{n} \cdot \vec{v}_2 \vec{S}_1 \cdot \vec{S}_1 \vec{v}_1 \cdot \vec{v}_2 + 3 \hat{n} \cdot \vec{S}_1 \vec{S}_1 \cdot \vec{v}_2 \vec{v}_1 \cdot \vec{v}_2 - 2 \hat{n} \cdot \vec{v}_1 \vec{S}_1 \cdot \vec{S}_1 \vec{v}_2 \cdot \vec{v}_2 \right) + \\
& \frac{1}{r^2} \left( - \left( \vec{a}_1 \cdot \vec{a}_2 \right) \left( \hat{n} \cdot \vec{S}_1 \right)^2 - \hat{n} \cdot \vec{v}_1 \vec{S}_1 \cdot \vec{a}_2 \hat{n} \cdot \vec{S}_1 - \hat{n} \cdot \vec{v}_1 \vec{S}_1 \cdot \vec{v}_2 \hat{n} \cdot \vec{S}_1 + 2 \hat{n} \cdot \vec{v}_2 \vec{S}_1 \cdot \vec{v}_2 \hat{n} \cdot \vec{S}_1 - \right. \\
& 2 \hat{n} \cdot \vec{S}_1 \vec{v}_1 \cdot \vec{a}_2 \hat{n} \cdot \vec{S}_1 - 2 \left( \vec{S}_1 \cdot \vec{v}_2 \right)^2 - 4 \left( \hat{n} \cdot \vec{v}_2 \right)^2 \vec{S}_1 \cdot \vec{S}_1 + 2 \hat{n} \cdot \vec{v}_1 \hat{n} \cdot \vec{v}_2 \vec{S}_1 \cdot \vec{S}_1 - 2 \hat{n} \cdot \vec{S}_1 \hat{n} \cdot \vec{v}_1 \vec{S}_1 \cdot \vec{v}_2 + \\
& 4 \hat{n} \cdot \vec{S}_1 \hat{n} \cdot \vec{v}_2 \vec{S}_1 \cdot \vec{v}_2 + 2 \hat{n} \cdot \vec{a}_2 \hat{n} \cdot \vec{v}_1 \vec{S}_1 \cdot \vec{S}_1 - 4 \left( \hat{n} \cdot \vec{v}_2 \right)^2 \vec{S}_1 \cdot \vec{S}_1 + 2 \hat{n} \cdot \vec{v}_1 \hat{n} \cdot \vec{v}_2 \vec{S}_1 \cdot \vec{S}_1 - \\
& \hat{n} \cdot \vec{S}_1 \hat{n} \cdot \vec{v}_1 \vec{S}_1 \cdot \vec{a}_2 + \vec{S}_1 \cdot \vec{v}_1 \vec{S}_1 \cdot \vec{a}_2 - \vec{a}_1 \cdot \vec{a}_2 \vec{S}_1 \cdot \vec{S}_1 + \vec{S}_1 \cdot \vec{a}_2 \vec{S}_1 \cdot \vec{v}_1 - \hat{n} \cdot \vec{S}_1 \hat{n} \cdot \vec{v}_1 \vec{S}_1 \cdot \vec{v}_2 + \\
& \left. 2 \hat{n} \cdot \vec{S}_1 \hat{n} \cdot \vec{v}_2 \vec{S}_1 \cdot \vec{v}_2 - 2 \vec{S}_1 \cdot \vec{v}_2 \vec{S}_1 \cdot \vec{v}_2 - 4 \vec{S}_1 \cdot \vec{S}_1 \vec{v}_1 \cdot \vec{a}_2 + 2 \vec{S}_1 \cdot \vec{S}_1 \vec{v}_2 \cdot \vec{v}_2 + 2 \vec{S}_1 \cdot \vec{S}_1 \vec{v}_2 \cdot \vec{v}_2 \right) \Bigg) m_2 C_{ES^2_1} \Bigg\}
\end{aligned}$$



{DiagS1CES2[2, 1, 8],

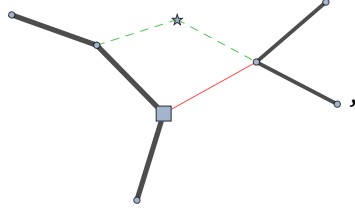

$$G^2 m_2 C_{ES^2 1} \left( \frac{1}{r^3} \left( -15 \vec{a}_1 \cdot \vec{v}_2 (\hat{n} \cdot \vec{S}_1)^2 \hat{n} \cdot \vec{v}_1 + 12 \vec{a}_1 \cdot \vec{v}_2 (\hat{n} \cdot \vec{S}_1)^2 \hat{n} \cdot \vec{v}_2 + \right. \right. \\
3 \vec{v}_1 \cdot \vec{a}_2 (\hat{n} \cdot \vec{S}_1)^2 \hat{n} \cdot \vec{v}_1 + 6 \vec{a}_1 \cdot \vec{v}_2 \hat{n} \cdot \vec{S}_1 \vec{S}_1 \cdot \vec{v}_1 - 6 \vec{a}_1 \cdot \vec{v}_2 \hat{n} \cdot \vec{S}_1 \vec{S}_1 \cdot \vec{v}_2 + 3 \vec{S}_1 \cdot \vec{S}_1 \vec{a}_1 \cdot \vec{v}_2 \hat{n} \cdot \vec{v}_1 - \\
2 \vec{S}_1 \cdot \vec{S}_1 \vec{a}_1 \cdot \vec{v}_2 \hat{n} \cdot \vec{v}_2 - \vec{S}_1 \cdot \vec{S}_1 \vec{v}_1 \cdot \vec{a}_2 \hat{n} \cdot \vec{v}_1 + 6 \vec{v}_1 \cdot \vec{v}_2 \hat{n} \cdot \vec{S}_1 \hat{n} \cdot \vec{S}_1 \hat{n} \cdot \vec{v}_1 - 2 \vec{S}_1 \cdot \vec{S}_1 \vec{v}_1 \cdot \vec{v}_2 \hat{n} \cdot \vec{v}_1 \Big) + \\
\frac{6 \vec{a}_1 \cdot \vec{v}_2 \hat{n} \cdot \vec{S}_1 \hat{n} \cdot \vec{S}_1 + 3 \vec{a}_1 \cdot \vec{a}_2 (\hat{n} \cdot \vec{S}_1)^2 - 2 \vec{S}_1 \cdot \vec{S}_1 \vec{a}_1 \cdot \vec{v}_2 - \vec{a}_1 \cdot \vec{a}_2 \vec{S}_1 \cdot \vec{S}_1}{r^2} + \frac{1}{r^4} \left( -3 (\vec{v}_1 \cdot \vec{v}_2)^2 (\hat{n} \cdot \vec{S}_1)^2 - \right. \\
15 \vec{v}_1 \cdot \vec{v}_2 (\hat{n} \cdot \vec{S}_1)^2 (\hat{n} \cdot \vec{v}_1)^2 + 18 \vec{v}_1 \cdot \vec{v}_2 (\hat{n} \cdot \vec{S}_1)^2 \hat{n} \cdot \vec{v}_1 \hat{n} \cdot \vec{v}_2 + 6 \vec{v}_1 \cdot \vec{v}_2 \hat{n} \cdot \vec{S}_1 \hat{n} \cdot \vec{v}_1 \vec{S}_1 \cdot \vec{v}_1 - \\
\left. \left. 6 \vec{v}_1 \cdot \vec{v}_2 \hat{n} \cdot \vec{S}_1 \hat{n} \cdot \vec{v}_1 \vec{S}_1 \cdot \vec{v}_2 + 3 \vec{S}_1 \cdot \vec{S}_1 \vec{v}_1 \cdot \vec{v}_2 (\hat{n} \cdot \vec{v}_1)^2 - 4 \vec{S}_1 \cdot \vec{S}_1 \vec{v}_1 \cdot \vec{v}_2 \hat{n} \cdot \vec{v}_1 \hat{n} \cdot \vec{v}_2 + \vec{S}_1 \cdot \vec{S}_1 (\vec{v}_1 \cdot \vec{v}_2)^2 \right) \right\}$$

{DiagS1CES2[2, 1, 9],

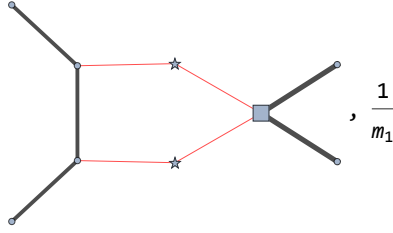

,  $\frac{1}{m_1}$

$$G^2 \left( \frac{1}{r^4} \left( 9 (\hat{n} \cdot \vec{S}_1)^2 (\hat{n} \cdot \vec{v}_2)^4 + \frac{3}{2} \vec{S}_1 \cdot \vec{S}_1 (\hat{n} \cdot \vec{v}_2)^4 - 72 (\hat{n} \cdot \vec{S}_1)^2 \hat{n} \cdot \vec{v}_1 (\hat{n} \cdot \vec{v}_2)^3 - 12 \hat{n} \cdot \vec{v}_1 \vec{S}_1 \cdot \vec{S}_1 (\hat{n} \cdot \vec{v}_2)^3 + \right. \right. \\
18 \hat{n} \cdot \vec{S}_1 \vec{S}_1 \cdot \vec{v}_1 (\hat{n} \cdot \vec{v}_2)^3 - 9 \hat{n} \cdot \vec{S}_1 \vec{S}_1 \cdot \vec{v}_2 (\hat{n} \cdot \vec{v}_2)^3 + 72 (\hat{n} \cdot \vec{S}_1)^2 (\hat{n} \cdot \vec{v}_1)^2 (\hat{n} \cdot \vec{v}_2)^2 + 3 (\vec{S}_1 \cdot \vec{v}_1)^2 (\hat{n} \cdot \vec{v}_2)^2 + \\
\frac{9}{4} (\vec{S}_1 \cdot \vec{v}_2)^2 (\hat{n} \cdot \vec{v}_2)^2 + 12 (\hat{n} \cdot \vec{v}_1)^2 \vec{S}_1 \cdot \vec{S}_1 (\hat{n} \cdot \vec{v}_2)^2 - 36 \hat{n} \cdot \vec{S}_1 \hat{n} \cdot \vec{v}_1 \vec{S}_1 \cdot \vec{v}_1 (\hat{n} \cdot \vec{v}_2)^2 + \\
54 \hat{n} \cdot \vec{S}_1 \hat{n} \cdot \vec{v}_1 \vec{S}_1 \cdot \vec{v}_2 (\hat{n} \cdot \vec{v}_2)^2 - 9 \vec{S}_1 \cdot \vec{v}_1 \vec{S}_1 \cdot \vec{v}_2 (\hat{n} \cdot \vec{v}_2)^2 - 9 (\hat{n} \cdot \vec{S}_1)^2 \vec{v}_1 \cdot \vec{v}_1 (\hat{n} \cdot \vec{v}_2)^2 - \\
2 \vec{S}_1 \cdot \vec{S}_1 \vec{v}_1 \cdot \vec{v}_1 (\hat{n} \cdot \vec{v}_2)^2 + 27 (\hat{n} \cdot \vec{S}_1)^2 \vec{v}_1 \cdot \vec{v}_2 (\hat{n} \cdot \vec{v}_2)^2 + 6 \vec{S}_1 \cdot \vec{S}_1 \vec{v}_1 \cdot \vec{v}_2 (\hat{n} \cdot \vec{v}_2)^2 - \\
9 (\hat{n} \cdot \vec{S}_1)^2 \vec{v}_2 \cdot \vec{v}_2 (\hat{n} \cdot \vec{v}_2)^2 - \frac{7}{4} \vec{S}_1 \cdot \vec{S}_1 \vec{v}_2 \cdot \vec{v}_2 (\hat{n} \cdot \vec{v}_2)^2 - 9 \hat{n} \cdot \vec{v}_1 (\vec{S}_1 \cdot \vec{v}_2)^2 \hat{n} \cdot \vec{v}_2 - \\
36 \hat{n} \cdot \vec{S}_1 (\hat{n} \cdot \vec{v}_1)^2 \vec{S}_1 \cdot \vec{v}_2 \hat{n} \cdot \vec{v}_2 + 12 \hat{n} \cdot \vec{v}_1 \vec{S}_1 \cdot \vec{v}_1 \vec{S}_1 \cdot \vec{v}_2 \hat{n} \cdot \vec{v}_2 + 6 \hat{n} \cdot \vec{S}_1 \vec{S}_1 \cdot \vec{v}_2 \vec{v}_1 \cdot \vec{v}_1 \hat{n} \cdot \vec{v}_2 - \\
36 (\hat{n} \cdot \vec{S}_1)^2 \hat{n} \cdot \vec{v}_1 \vec{v}_1 \cdot \vec{v}_2 \hat{n} \cdot \vec{v}_2 - 8 \hat{n} \cdot \vec{v}_1 \vec{S}_1 \cdot \vec{S}_1 \vec{v}_1 \cdot \vec{v}_2 \hat{n} \cdot \vec{v}_2 + 12 \hat{n} \cdot \vec{S}_1 \vec{S}_1 \cdot \vec{v}_1 \vec{v}_1 \cdot \vec{v}_2 \hat{n} \cdot \vec{v}_2 - \\
18 \hat{n} \cdot \vec{S}_1 \vec{S}_1 \cdot \vec{v}_2 \vec{v}_1 \cdot \vec{v}_2 \hat{n} \cdot \vec{v}_2 + 18 (\hat{n} \cdot \vec{S}_1)^2 \hat{n} \cdot \vec{v}_1 \vec{v}_2 \cdot \vec{v}_2 \hat{n} \cdot \vec{v}_2 + 5 \hat{n} \cdot \vec{v}_1 \vec{S}_1 \cdot \vec{S}_1 \vec{v}_2 \cdot \vec{v}_2 \hat{n} \cdot \vec{v}_2 - \\
6 \hat{n} \cdot \vec{S}_1 \vec{S}_1 \cdot \vec{v}_1 \vec{v}_2 \cdot \vec{v}_2 \hat{n} \cdot \vec{v}_2 + 6 \hat{n} \cdot \vec{S}_1 \vec{S}_1 \cdot \vec{v}_2 \vec{v}_2 \cdot \vec{v}_2 \hat{n} \cdot \vec{v}_2 + 3 (\hat{n} \cdot \vec{v}_1)^2 (\vec{S}_1 \cdot \vec{v}_2)^2 + \\
3 (\hat{n} \cdot \vec{S}_1)^2 (\vec{v}_1 \cdot \vec{v}_2)^2 + \vec{S}_1 \cdot \vec{S}_1 (\vec{v}_1 \cdot \vec{v}_2)^2 + \frac{3}{2} (\hat{n} \cdot \vec{S}_1)^2 (\vec{v}_2 \cdot \vec{v}_2)^2 + \frac{1}{4} \vec{S}_1 \cdot \vec{S}_1 (\vec{v}_2 \cdot \vec{v}_2)^2 - \\
\frac{3}{4} (\vec{S}_1 \cdot \vec{v}_2)^2 \vec{v}_1 \cdot \vec{v}_1 + \frac{9}{4} (\vec{S}_1 \cdot \vec{v}_2)^2 \vec{v}_1 \cdot \vec{v}_2 + 12 \hat{n} \cdot \vec{S}_1 \hat{n} \cdot \vec{v}_1 \vec{S}_1 \cdot \vec{v}_2 \vec{v}_1 \cdot \vec{v}_2 - 3 \vec{S}_1 \cdot \vec{v}_1 \vec{S}_1 \cdot \vec{v}_2 \vec{v}_1 \cdot \vec{v}_2 - \\
\frac{3}{4} (\vec{S}_1 \cdot \vec{v}_2)^2 \vec{v}_2 \cdot \vec{v}_2 - (\hat{n} \cdot \vec{v}_1)^2 \vec{S}_1 \cdot \vec{S}_1 \vec{v}_2 \cdot \vec{v}_2 - 6 \hat{n} \cdot \vec{S}_1 \hat{n} \cdot \vec{v}_1 \vec{S}_1 \cdot \vec{v}_2 \vec{v}_2 \cdot \vec{v}_2 + \frac{3}{2} \vec{S}_1 \cdot \vec{v}_1 \vec{S}_1 \cdot \vec{v}_2 \vec{v}_2 \cdot \vec{v}_2 + \left. \right)$$

$$\begin{aligned}
& \frac{1}{4} \vec{S}_1 \cdot \vec{S}_1 \vec{v}_1 \cdot \vec{v}_1 \vec{v}_2 \cdot \vec{v}_2 - 3 \left( \hat{n} \cdot \vec{S}_1 \right)^2 \vec{v}_1 \cdot \vec{v}_2 \vec{v}_2 \cdot \vec{v}_2 - \frac{5}{4} \vec{S}_1 \cdot \vec{S}_1 \vec{v}_1 \cdot \vec{v}_2 \vec{v}_2 \cdot \vec{v}_2 \Big) + \frac{1}{r^3} \\
& \left( 18 \hat{n} \cdot \vec{S}_1 \hat{n} \cdot \vec{S}_1 (\hat{n} \cdot \vec{v}_2)^3 + 6 \vec{S}_1 \cdot \vec{S}_1 (\hat{n} \cdot \vec{v}_2)^3 - \vec{S}_1^2 (\hat{n} \cdot \vec{v}_2)^3 - 9 \hat{n} \cdot \vec{a}_1 (\hat{n} \cdot \vec{S}_1)^2 (\hat{n} \cdot \vec{v}_2)^2 + \right. \\
& 9 \hat{n} \cdot \vec{a}_2 (\hat{n} \cdot \vec{S}_1)^2 (\hat{n} \cdot \vec{v}_2)^2 - 36 \hat{n} \cdot \vec{S}_1 \hat{n} \cdot \vec{S}_1 \hat{n} \cdot \vec{v}_1 (\hat{n} \cdot \vec{v}_2)^2 + 6 \hat{n} \cdot \vec{S}_1 \vec{S}_1 \cdot \vec{v}_1 (\hat{n} \cdot \vec{v}_2)^2 - \\
& 9 \hat{n} \cdot \vec{S}_1 \vec{S}_1 \cdot \vec{v}_2 (\hat{n} \cdot \vec{v}_2)^2 - 12 \hat{n} \cdot \vec{v}_1 \vec{S}_1 \cdot \vec{S}_1 (\hat{n} \cdot \vec{v}_2)^2 + 3 \hat{n} \cdot \vec{S}_1 \vec{S}_1 \cdot \vec{a}_1 (\hat{n} \cdot \vec{v}_2)^2 - 3 \hat{n} \cdot \vec{S}_1 \vec{S}_1 \cdot \vec{a}_2 (\hat{n} \cdot \vec{v}_2)^2 - \\
& 2 \hat{n} \cdot \vec{a}_1 \vec{S}_1 \cdot \vec{S}_1 (\hat{n} \cdot \vec{v}_2)^2 + 2 \hat{n} \cdot \vec{a}_2 \vec{S}_1 \cdot \vec{S}_1 (\hat{n} \cdot \vec{v}_2)^2 + 6 \hat{n} \cdot \vec{S}_1 \vec{S}_1 \cdot \vec{v}_1 (\hat{n} \cdot \vec{v}_2)^2 - 9 \hat{n} \cdot \vec{S}_1 \vec{S}_1 \cdot \vec{v}_2 (\hat{n} \cdot \vec{v}_2)^2 + \\
& 2 \hat{n} \cdot \vec{v}_1 \vec{S}_1^2 (\hat{n} \cdot \vec{v}_2)^2 - 18 \hat{n} \cdot \vec{a}_2 (\hat{n} \cdot \vec{S}_1)^2 \hat{n} \cdot \vec{v}_1 \hat{n} \cdot \vec{v}_2 + 12 \hat{n} \cdot \vec{S}_1 \hat{n} \cdot \vec{v}_1 \vec{S}_1 \cdot \vec{v}_2 \hat{n} \cdot \vec{v}_2 + \\
& 3 (\hat{n} \cdot \vec{S}_1)^2 \vec{a}_1 \cdot \vec{v}_2 \hat{n} \cdot \vec{v}_2 + 6 \hat{n} \cdot \vec{S}_1 \hat{n} \cdot \vec{v}_1 \vec{S}_1 \cdot \vec{a}_2 \hat{n} \cdot \vec{v}_2 - 4 \hat{n} \cdot \vec{a}_2 \hat{n} \cdot \vec{v}_1 \vec{S}_1 \cdot \vec{S}_1 \hat{n} \cdot \vec{v}_2 + \vec{a}_1 \cdot \vec{v}_2 \vec{S}_1 \cdot \vec{S}_1 \hat{n} \cdot \vec{v}_2 + \\
& 6 \hat{n} \cdot \vec{a}_2 \hat{n} \cdot \vec{S}_1 \vec{S}_1 \cdot \vec{v}_1 \hat{n} \cdot \vec{v}_2 - 3 \vec{S}_1^2 \cdot \vec{v}_2 \vec{S}_1 \cdot \vec{v}_1 \hat{n} \cdot \vec{v}_2 - \frac{3}{2} \vec{S}_1 \cdot \vec{a}_2 \vec{S}_1 \cdot \vec{v}_1 \hat{n} \cdot \vec{v}_2 + 6 \hat{n} \cdot \vec{a}_1 \hat{n} \cdot \vec{S}_1 \vec{S}_1 \cdot \vec{v}_2 \hat{n} \cdot \vec{v}_2 - \\
& 6 \hat{n} \cdot \vec{a}_2 \hat{n} \cdot \vec{S}_1 \vec{S}_1 \cdot \vec{v}_2 \hat{n} \cdot \vec{v}_2 + 12 \hat{n} \cdot \vec{S}_1 \hat{n} \cdot \vec{v}_1 \vec{S}_1 \cdot \vec{v}_2 \hat{n} \cdot \vec{v}_2 - 3 \vec{S}_1^2 \cdot \vec{v}_1 \vec{S}_1 \cdot \vec{v}_2 \hat{n} \cdot \vec{v}_2 + \frac{9}{2} \vec{S}_1 \cdot \vec{v}_2 \vec{S}_1 \cdot \vec{v}_2 \hat{n} \cdot \vec{v}_2 - \\
& \frac{3}{2} \vec{S}_1 \cdot \vec{a}_1 \vec{S}_1 \cdot \vec{v}_2 \hat{n} \cdot \vec{v}_2 + \frac{3}{2} \vec{S}_1 \cdot \vec{a}_2 \vec{S}_1 \cdot \vec{v}_2 \hat{n} \cdot \vec{v}_2 + 3 (\hat{n} \cdot \vec{S}_1)^2 \vec{v}_1 \cdot \vec{a}_2 \hat{n} \cdot \vec{v}_2 + \vec{S}_1 \cdot \vec{S}_1 \vec{v}_1 \cdot \vec{a}_2 \hat{n} \cdot \vec{v}_2 + \\
& 12 \hat{n} \cdot \vec{S}_1 \hat{n} \cdot \vec{S}_1 \vec{v}_1 \cdot \vec{v}_2 \hat{n} \cdot \vec{v}_2 + 6 \vec{S}_1 \cdot \vec{S}_1 \vec{v}_1 \cdot \vec{v}_2 \hat{n} \cdot \vec{v}_2 - \frac{1}{2} \vec{S}_1 \cdot \vec{S}_1 \vec{v}_2 \cdot \vec{a}_2 \hat{n} \cdot \vec{v}_2 - 6 \hat{n} \cdot \vec{S}_1 \hat{n} \cdot \vec{S}_1 \vec{v}_2 \cdot \vec{v}_2 \hat{n} \cdot \vec{v}_2 - \\
& \frac{9}{2} \vec{S}_1 \cdot \vec{S}_1 \vec{v}_2 \cdot \vec{v}_2 \hat{n} \cdot \vec{v}_2 - \vec{v}_1 \cdot \vec{v}_2 \vec{S}_1^2 \hat{n} \cdot \vec{v}_2 + \vec{v}_2 \cdot \vec{v}_2 \vec{S}_1^2 \hat{n} \cdot \vec{v}_2 - \frac{3}{4} \hat{n} \cdot \vec{a}_1 (\vec{S}_1 \cdot \vec{v}_2)^2 + \frac{3}{4} \hat{n} \cdot \vec{a}_2 (\vec{S}_1 \cdot \vec{v}_2)^2 + \\
& 6 \hat{n} \cdot \vec{a}_2 \hat{n} \cdot \vec{S}_1 \hat{n} \cdot \vec{v}_1 \vec{S}_1 \cdot \vec{v}_2 - 3 \hat{n} \cdot \vec{v}_1 \vec{S}_1 \cdot \vec{v}_2 \vec{S}_1 \cdot \vec{v}_2 - \frac{3}{2} \hat{n} \cdot \vec{S}_1 \vec{a}_1 \cdot \vec{v}_2 \vec{S}_1 \cdot \vec{v}_2 - \frac{3}{2} \hat{n} \cdot \vec{v}_1 \vec{S}_1 \cdot \vec{a}_2 \vec{S}_1 \cdot \vec{v}_2 - \\
& \frac{3}{2} \hat{n} \cdot \vec{a}_2 \vec{S}_1 \cdot \vec{v}_1 \vec{S}_1 \cdot \vec{v}_2 - \frac{3}{2} \hat{n} \cdot \vec{S}_1 \vec{S}_1 \cdot \vec{v}_2 \vec{v}_1 \cdot \vec{a}_2 + 3 \hat{n} \cdot \vec{a}_2 (\hat{n} \cdot \vec{S}_1)^2 \vec{v}_1 \cdot \vec{v}_2 - 3 \hat{n} \cdot \vec{S}_1 \vec{S}_1 \cdot \vec{v}_2 \vec{v}_1 \cdot \vec{v}_2 - \\
& \frac{3}{2} \hat{n} \cdot \vec{S}_1 \vec{S}_1 \cdot \vec{a}_2 \vec{v}_1 \cdot \vec{v}_2 + \hat{n} \cdot \vec{a}_2 \vec{S}_1 \cdot \vec{S}_1 \vec{v}_1 \cdot \vec{v}_2 - 3 \hat{n} \cdot \vec{S}_1 \vec{S}_1 \cdot \vec{v}_2 \vec{v}_1 \cdot \vec{v}_2 + \frac{1}{2} \hat{n} \cdot \vec{v}_1 \vec{S}_1 \cdot \vec{S}_1 \vec{v}_2 \cdot \vec{a}_2 - \\
& 3 \hat{n} \cdot \vec{a}_2 (\hat{n} \cdot \vec{S}_1)^2 \vec{v}_2 \cdot \vec{v}_2 + \frac{3}{2} \hat{n} \cdot \vec{S}_1 \vec{S}_1 \cdot \vec{v}_2 \vec{v}_2 \cdot \vec{v}_2 + 3 \hat{n} \cdot \vec{v}_1 \vec{S}_1 \cdot \vec{S}_1 \vec{v}_2 \cdot \vec{v}_2 + \frac{3}{2} \hat{n} \cdot \vec{S}_1 \vec{S}_1 \cdot \vec{a}_2 \vec{v}_2 \cdot \vec{v}_2 + \\
& \frac{1}{4} \hat{n} \cdot \vec{a}_1 \vec{S}_1 \cdot \vec{S}_1 \vec{v}_2 \cdot \vec{v}_2 - \frac{3}{4} \hat{n} \cdot \vec{a}_2 \vec{S}_1 \cdot \vec{S}_1 \vec{v}_2 \cdot \vec{v}_2 + \frac{3}{2} \hat{n} \cdot \vec{S}_1 \vec{S}_1 \cdot \vec{v}_2 \vec{v}_2 \cdot \vec{v}_2 - \hat{n} \cdot \vec{v}_1 \vec{v}_2 \cdot \vec{v}_2 \vec{S}_1^2 \Big) + \frac{1}{r^2} \\
& \left( \frac{3}{2} (\hat{n} \cdot \vec{S}_1)^2 (\hat{n} \cdot \vec{a}_2)^2 + \frac{1}{2} \vec{S}_1 \cdot \vec{S}_1 (\hat{n} \cdot \vec{a}_2)^2 + 6 \hat{n} \cdot \vec{S}_1 \hat{n} \cdot \vec{S}_1 \hat{n} \cdot \vec{v}_2 \hat{n} \cdot \vec{a}_2 - \frac{3}{2} \hat{n} \cdot \vec{S}_1 \vec{S}_1 \cdot \vec{v}_2 \hat{n} \cdot \vec{a}_2 + \right. \\
& 3 \hat{n} \cdot \vec{v}_2 \vec{S}_1 \cdot \vec{S}_1 \hat{n} \cdot \vec{a}_2 - \frac{3}{2} \hat{n} \cdot \vec{S}_1 \vec{S}_1 \cdot \vec{a}_2 \hat{n} \cdot \vec{a}_2 - \frac{3}{2} \hat{n} \cdot \vec{S}_1 \vec{S}_1 \cdot \vec{v}_2 \hat{n} \cdot \vec{a}_2 - \frac{1}{2} \hat{n} \cdot \vec{v}_2 \vec{S}_1^2 \hat{n} \cdot \vec{a}_2 + 3 \left( \hat{n} \cdot \vec{S}_1 \right)^2 (\hat{n} \cdot \vec{v}_2)^2 + \\
& 3 \hat{n} \cdot \vec{S}_1 \hat{n} \cdot \vec{S}_1 (\hat{n} \cdot \vec{v}_2)^2 + \frac{3}{4} \left( \frac{1}{\vec{S}_1 \cdot \vec{v}_2} \right)^2 + \frac{3}{8} (\vec{S}_1 \cdot \vec{a}_2)^2 + \frac{3}{2} (\hat{n} \cdot \vec{v}_2)^2 \frac{1}{\vec{S}_1 \cdot \vec{S}_1} - \frac{3}{2} \hat{n} \cdot \vec{S}_1 \hat{n} \cdot \vec{v}_2 \vec{S}_1 \cdot \vec{a}_2 - \\
& 3 \hat{n} \cdot \vec{S}_1 \hat{n} \cdot \vec{v}_2 \vec{S}_1 \cdot \vec{v}_2 - \frac{3}{2} \hat{n} \cdot \vec{S}_1 \hat{n} \cdot \vec{v}_2 \vec{S}_1 \cdot \vec{v}_2 + \frac{3}{2} (\hat{n} \cdot \vec{v}_2)^2 \vec{S}_1 \cdot \vec{S}_1 - \frac{3}{2} \hat{n} \cdot \vec{S}_1 \hat{n} \cdot \vec{v}_2 \vec{S}_1 \cdot \vec{a}_2 + \frac{3}{4} \vec{S}_1 \cdot \vec{v}_2 \vec{S}_1 \cdot \vec{a}_2 - \\
& \frac{1}{8} \vec{a}_2 \cdot \vec{a}_2 \vec{S}_1 \cdot \vec{S}_1 - \frac{3}{2} \hat{n} \cdot \vec{S}_1 \hat{n} \cdot \vec{v}_2 \vec{S}_1 \cdot \vec{v}_2 + \frac{3}{4} \vec{S}_1 \cdot \vec{a}_2 \vec{S}_1 \cdot \vec{v}_2 + \frac{3}{4} \vec{S}_1 \cdot \vec{v}_2 \vec{S}_1 \cdot \vec{v}_2 - \frac{3}{2} \vec{S}_1 \cdot \vec{S}_1 \vec{v}_2 \cdot \vec{a}_2 - \\
& \left. \frac{3}{4} \vec{S}_1 \cdot \vec{S}_1 \vec{v}_2 \cdot \vec{v}_2 - \frac{3}{4} \vec{S}_1 \cdot \vec{S}_1 \vec{v}_2 \cdot \vec{v}_2 + \frac{1}{2} \vec{v}_2 \cdot \vec{a}_2 \vec{S}_1^2 - \frac{1}{4} (\hat{n} \cdot \vec{v}_2)^2 \vec{S}_1^2 + \frac{1}{4} \vec{v}_2 \cdot \vec{v}_2 \vec{S}_1^2 \right) \Big) m_{\text{ES}^2}^2 \}
\end{aligned}$$

{DiagS1CES2[2, 1, 10],

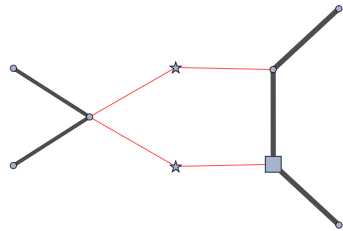

,



$$\left. \begin{aligned} & \frac{1}{4} \hat{n} \cdot \vec{a_1} \vec{S_1} \cdot \vec{S_1} \vec{v_1} \cdot \vec{v_1} - \frac{1}{2} \hat{n} \cdot \vec{S_1} \vec{S_1} \cdot \vec{v_1} \vec{v_1} \cdot \vec{v_1} + \frac{1}{4} \hat{n} \cdot \vec{S_1} \vec{S_1} \cdot \vec{v_2} \vec{v_1} \cdot \vec{v_1} - \frac{3}{4} \hat{n} \cdot \vec{a_1} \left( \hat{n} \cdot \vec{S_1} \right)^2 \vec{v_1} \cdot \vec{v_2} + \\ & 2 \hat{n} \cdot \vec{S_1} \hat{n} \cdot \vec{S_1} \hat{n} \cdot \vec{v_2} \vec{v_1} \cdot \vec{v_2} + \frac{1}{2} \hat{n} \cdot \vec{S_1} \vec{S_1} \cdot \vec{v_1} \vec{v_1} \cdot \vec{v_2} - \frac{1}{2} \hat{n} \cdot \vec{S_1} \vec{S_1} \cdot \vec{v_2} \vec{v_1} \cdot \vec{v_2} + \hat{n} \cdot \vec{v_2} \vec{S_1} \cdot \vec{S_1} \vec{v_1} \cdot \vec{v_2} + \\ & \frac{1}{4} \hat{n} \cdot \vec{S_1} \vec{S_1} \cdot \vec{a_1} \vec{v_1} \cdot \vec{v_2} - \frac{1}{4} \hat{n} \cdot \vec{a_1} \vec{S_1} \cdot \vec{S_1} \vec{v_1} \cdot \vec{v_2} + \frac{1}{2} \hat{n} \cdot \vec{S_1} \vec{S_1} \cdot \vec{v_1} \vec{v_1} \cdot \vec{v_2} - \frac{1}{2} \hat{n} \cdot \vec{S_1} \vec{S_1} \cdot \vec{v_2} \vec{v_1} \cdot \vec{v_2} \Big) + \frac{1}{r^4} \\ & \left( \frac{15}{8} \left( \hat{n} \cdot \vec{S_1} \right)^2 \left( \hat{n} \cdot \vec{v_1} \right)^4 + \frac{3}{8} \vec{S_1} \cdot \vec{S_1} \left( \hat{n} \cdot \vec{v_1} \right)^4 - 18 \left( \hat{n} \cdot \vec{S_1} \right)^2 \hat{n} \cdot \vec{v_2} \left( \hat{n} \cdot \vec{v_1} \right)^3 - 3 \hat{n} \cdot \vec{v_2} \vec{S_1} \cdot \vec{S_1} \left( \hat{n} \cdot \vec{v_1} \right)^3 - \\ & \frac{3}{2} \hat{n} \cdot \vec{S_1} \vec{S_1} \cdot \vec{v_1} \left( \hat{n} \cdot \vec{v_1} \right)^3 + \frac{9}{2} \hat{n} \cdot \vec{S_1} \vec{S_1} \cdot \vec{v_2} \left( \hat{n} \cdot \vec{v_1} \right)^3 + 18 \left( \hat{n} \cdot \vec{S_1} \right)^2 \left( \hat{n} \cdot \vec{v_2} \right)^2 \left( \hat{n} \cdot \vec{v_1} \right)^2 + \frac{1}{4} \left( \vec{S_1} \cdot \vec{v_1} \right)^2 \left( \hat{n} \cdot \vec{v_1} \right)^2 + \\ & \frac{3}{4} \left( \vec{S_1} \cdot \vec{v_2} \right)^2 \left( \hat{n} \cdot \vec{v_1} \right)^2 + 3 \left( \hat{n} \cdot \vec{v_2} \right)^2 \vec{S_1} \cdot \vec{S_1} \left( \hat{n} \cdot \vec{v_1} \right)^2 + \frac{21}{2} \hat{n} \cdot \vec{S_1} \hat{n} \cdot \vec{v_2} \vec{S_1} \cdot \vec{v_1} \left( \hat{n} \cdot \vec{v_1} \right)^2 - \\ & 9 \hat{n} \cdot \vec{S_1} \hat{n} \cdot \vec{v_2} \vec{S_1} \cdot \vec{v_2} \left( \hat{n} \cdot \vec{v_1} \right)^2 - \frac{7}{4} \vec{S_1} \cdot \vec{v_1} \vec{S_1} \cdot \vec{v_2} \left( \hat{n} \cdot \vec{v_1} \right)^2 - \frac{9}{4} \left( \hat{n} \cdot \vec{S_1} \right)^2 \vec{v_1} \cdot \vec{v_1} \left( \hat{n} \cdot \vec{v_1} \right)^2 - \\ & \frac{1}{2} \vec{S_1} \cdot \vec{S_1} \vec{v_1} \cdot \vec{v_1} \left( \hat{n} \cdot \vec{v_1} \right)^2 + \frac{27}{4} \left( \hat{n} \cdot \vec{S_1} \right)^2 \vec{v_1} \cdot \vec{v_2} \left( \hat{n} \cdot \vec{v_1} \right)^2 + \frac{3}{2} \vec{S_1} \cdot \vec{S_1} \vec{v_1} \cdot \vec{v_2} \left( \hat{n} \cdot \vec{v_1} \right)^2 - \\ & \frac{9}{4} \left( \hat{n} \cdot \vec{S_1} \right)^2 \vec{v_2} \cdot \vec{v_2} \left( \hat{n} \cdot \vec{v_1} \right)^2 - \frac{1}{2} \vec{S_1} \cdot \vec{S_1} \vec{v_2} \cdot \vec{v_2} \left( \hat{n} \cdot \vec{v_1} \right)^2 - \hat{n} \cdot \vec{v_2} \left( \vec{S_1} \cdot \vec{v_1} \right)^2 \hat{n} \cdot \vec{v_1} - 6 \hat{n} \cdot \vec{S_1} \left( \hat{n} \cdot \vec{v_2} \right)^2 \vec{S_1} \cdot \vec{v_1} \hat{n} \cdot \vec{v_1} + \\ & 2 \hat{n} \cdot \vec{v_2} \vec{S_1} \cdot \vec{v_1} \vec{S_1} \cdot \vec{v_2} \hat{n} \cdot \vec{v_1} + \frac{9}{2} \left( \hat{n} \cdot \vec{S_1} \right)^2 \hat{n} \cdot \vec{v_2} \vec{v_1} \cdot \vec{v_1} \hat{n} \cdot \vec{v_1} + \hat{n} \cdot \vec{v_2} \vec{S_1} \cdot \vec{S_1} \vec{v_1} \cdot \vec{v_1} \hat{n} \cdot \vec{v_1} + \\ & \frac{3}{2} \hat{n} \cdot \vec{S_1} \vec{S_1} \cdot \vec{v_1} \vec{v_1} \cdot \vec{v_1} \hat{n} \cdot \vec{v_1} - \frac{3}{2} \hat{n} \cdot \vec{S_1} \vec{S_1} \cdot \vec{v_2} \vec{v_1} \cdot \vec{v_1} \hat{n} \cdot \vec{v_1} - 9 \left( \hat{n} \cdot \vec{S_1} \right)^2 \hat{n} \cdot \vec{v_2} \vec{v_1} \cdot \vec{v_2} \hat{n} \cdot \vec{v_1} - \\ & 2 \hat{n} \cdot \vec{v_2} \vec{S_1} \cdot \vec{S_1} \vec{v_1} \cdot \vec{v_2} \hat{n} \cdot \vec{v_1} - \frac{7}{2} \hat{n} \cdot \vec{S_1} \vec{S_1} \cdot \vec{v_1} \vec{v_1} \cdot \vec{v_2} \hat{n} \cdot \vec{v_1} + 3 \hat{n} \cdot \vec{S_1} \vec{S_1} \cdot \vec{v_2} \vec{v_1} \cdot \vec{v_2} \hat{n} \cdot \vec{v_1} + \hat{n} \cdot \vec{S_1} \vec{S_1} \cdot \vec{v_1} \vec{v_2} \cdot \vec{v_2} \hat{n} \cdot \vec{v_1} - \\ & \frac{3}{8} \left( \hat{n} \cdot \vec{S_1} \right)^2 \left( \vec{v_1} \cdot \vec{v_1} \right)^2 + \frac{1}{8} \vec{S_1} \cdot \vec{S_1} \left( \vec{v_1} \cdot \vec{v_1} \right)^2 + \frac{3}{4} \left( \hat{n} \cdot \vec{S_1} \right)^2 \left( \vec{v_1} \cdot \vec{v_2} \right)^2 + \frac{1}{4} \vec{S_1} \cdot \vec{S_1} \left( \vec{v_1} \cdot \vec{v_2} \right)^2 - \frac{1}{4} \left( \vec{S_1} \cdot \vec{v_1} \right)^2 \vec{v_1} \cdot \vec{v_1} - \\ & \hat{n} \cdot \vec{S_1} \hat{n} \cdot \vec{v_2} \vec{S_1} \cdot \vec{v_1} \vec{v_1} \cdot \vec{v_1} + \frac{1}{4} \vec{S_1} \cdot \vec{v_1} \vec{S_1} \cdot \vec{v_2} \vec{v_1} \cdot \vec{v_1} + \frac{1}{4} \left( \vec{S_1} \cdot \vec{v_1} \right)^2 \vec{v_1} \cdot \vec{v_2} + 2 \hat{n} \cdot \vec{S_1} \hat{n} \cdot \vec{v_2} \vec{S_1} \cdot \vec{v_1} \vec{v_1} \cdot \vec{v_2} - \\ & \frac{1}{2} \vec{S_1} \cdot \vec{v_1} \vec{S_1} \cdot \vec{v_2} \vec{v_1} \cdot \vec{v_2} - \frac{3}{4} \left( \hat{n} \cdot \vec{S_1} \right)^2 \vec{v_1} \cdot \vec{v_1} \vec{v_1} \cdot \vec{v_2} - \frac{1}{4} \vec{S_1} \cdot \vec{S_1} \vec{v_1} \cdot \vec{v_1} \vec{v_1} \cdot \vec{v_2} \Big) \left. m_2 C_{\text{ES}^2} \right\} \end{aligned} \right\}$$

$\{\text{DiagS1CES2}[2, 1, 11],$

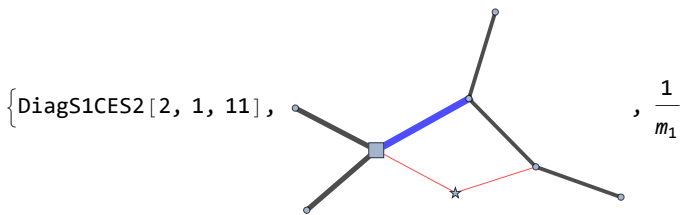

$, \frac{1}{m_1}$

$$\begin{aligned} G^2 \left( \frac{1}{r^3} \right. & \left( -8 \vec{S_1} \cdot \vec{S_1} \left( \hat{n} \cdot \vec{v_2} \right)^3 + 4 \hat{n} \cdot \vec{S_1} \vec{S_1} \cdot \vec{v_2} \left( \hat{n} \cdot \vec{v_2} \right)^2 + 4 \hat{n} \cdot \vec{S_1} \vec{S_1} \cdot \vec{a_2} \left( \hat{n} \cdot \vec{v_2} \right)^2 - 8 \hat{n} \cdot \vec{a_2} \vec{S_1} \cdot \vec{S_1} \left( \hat{n} \cdot \vec{v_2} \right)^2 + \right. \\ & 4 \hat{n} \cdot \vec{S_1} \vec{S_1} \cdot \vec{v_2} \left( \hat{n} \cdot \vec{v_2} \right)^2 + 4 \hat{n} \cdot \vec{a_2} \hat{n} \cdot \vec{S_1} \vec{S_1} \cdot \vec{v_2} \hat{n} \cdot \vec{v_2} - 4 \vec{S_1} \cdot \vec{v_2} \vec{S_1} \cdot \vec{v_2} \hat{n} \cdot \vec{v_2} - 3 \vec{S_1} \cdot \vec{a_2} \vec{S_1} \cdot \vec{v_2} \hat{n} \cdot \vec{v_2} - 8 \left( \hat{n} \cdot \vec{S_1} \right)^2 \\ & \vec{v_2} \cdot \vec{a_2} \hat{n} \cdot \vec{v_2} + 3 \vec{S_1} \cdot \vec{S_1} \vec{v_2} \cdot \vec{a_2} \hat{n} \cdot \vec{v_2} - 8 \hat{n} \cdot \vec{S_1} \hat{n} \cdot \vec{S_1} \vec{v_2} \cdot \vec{v_2} \hat{n} \cdot \vec{v_2} + 6 \vec{S_1} \cdot \vec{S_1} \vec{v_2} \cdot \vec{v_2} \hat{n} \cdot \vec{v_2} - \hat{n} \cdot \vec{a_2} \left( \vec{S_1} \cdot \vec{v_2} \right)^2 + \\ & \left. 4 \hat{n} \cdot \vec{S_1} \vec{S_1} \cdot \vec{v_2} \vec{v_2} \cdot \vec{a_2} + \hat{n} \cdot \vec{S_1} \vec{S_1} \cdot \vec{v_2} \vec{v_2} \cdot \vec{v_2} - 2 \hat{n} \cdot \vec{S_1} \vec{S_1} \cdot \vec{a_2} \vec{v_2} \cdot \vec{v_2} + 3 \hat{n} \cdot \vec{a_2} \vec{S_1} \cdot \vec{S_1} \vec{v_2} \cdot \vec{v_2} + \hat{n} \cdot \vec{S_1} \vec{S_1} \cdot \vec{v_2} \vec{v_2} \cdot \vec{v_2} \right) + \\ & \frac{1}{r^4} \left( -6 \vec{S_1} \cdot \vec{S_1} \left( \hat{n} \cdot \vec{v_2} \right)^4 + 24 \hat{n} \cdot \vec{v_1} \vec{S_1} \cdot \vec{S_1} \left( \hat{n} \cdot \vec{v_2} \right)^3 + 6 \hat{n} \cdot \vec{S_1} \vec{S_1} \cdot \vec{v_2} \left( \hat{n} \cdot \vec{v_2} \right)^3 - \frac{5}{2} \left( \vec{S_1} \cdot \vec{v_2} \right)^2 \left( \hat{n} \cdot \vec{v_2} \right)^2 - \right. \\ & 24 \hat{n} \cdot \vec{S_1} \hat{n} \cdot \vec{v_1} \vec{S_1} \cdot \vec{v_2} \left( \hat{n} \cdot \vec{v_2} \right)^2 + 4 \vec{S_1} \cdot \vec{v_1} \vec{S_1} \cdot \vec{v_2} \left( \hat{n} \cdot \vec{v_2} \right)^2 - 12 \vec{S_1} \cdot \vec{S_1} \vec{v_1} \cdot \vec{v_2} \left( \hat{n} \cdot \vec{v_2} \right)^2 - \\ & \left. 6 \left( \hat{n} \cdot \vec{S_1} \right)^2 \vec{v_2} \cdot \vec{v_2} \left( \hat{n} \cdot \vec{v_2} \right)^2 + \frac{11}{2} \vec{S_1} \cdot \vec{S_1} \vec{v_2} \cdot \vec{v_2} \left( \hat{n} \cdot \vec{v_2} \right)^2 + 8 \hat{n} \cdot \vec{v_1} \left( \vec{S_1} \cdot \vec{v_2} \right)^2 \hat{n} \cdot \vec{v_2} + 8 \hat{n} \cdot \vec{S_1} \vec{S_1} \cdot \vec{v_2} \vec{v_1} \cdot \vec{v_2} \hat{n} \cdot \vec{v_2} + \right. \end{aligned}$$

$$\begin{aligned} & 24 \left( \hat{n} \cdot \vec{S}_1 \right)^2 \hat{n} \cdot \vec{v}_1 \vec{v}_2 \cdot \vec{v}_2 \hat{n} \cdot \vec{v}_2 - 12 \hat{n} \cdot \vec{v}_1 \vec{S}_1 \cdot \vec{S}_1 \vec{v}_2 \cdot \vec{v}_2 \hat{n} \cdot \vec{v}_2 - 8 \hat{n} \cdot \vec{S}_1 \vec{S}_1 \cdot \vec{v}_1 \vec{v}_2 \cdot \vec{v}_2 \hat{n} \cdot \vec{v}_2 + \\ & 2 \hat{n} \cdot \vec{S}_1 \vec{S}_1 \cdot \vec{v}_2 \vec{v}_2 \cdot \vec{v}_2 \hat{n} \cdot \vec{v}_2 - \frac{1}{2} \vec{S}_1 \cdot \vec{S}_1 \left( \vec{v}_2 \cdot \vec{v}_2 \right)^2 - 2 \left( \vec{S}_1 \cdot \vec{v}_2 \right)^2 \vec{v}_1 \cdot \vec{v}_2 - \frac{1}{2} \left( \vec{S}_1 \cdot \vec{v}_2 \right)^2 \vec{v}_2 \cdot \vec{v}_2 - \\ & 4 \hat{n} \cdot \vec{S}_1 \hat{n} \cdot \vec{v}_1 \vec{S}_1 \cdot \vec{v}_2 \vec{v}_2 \cdot \vec{v}_2 + \vec{S}_1 \cdot \vec{v}_1 \vec{S}_1 \cdot \vec{v}_2 \vec{v}_2 \cdot \vec{v}_2 - 4 \left( \hat{n} \cdot \vec{S}_1 \right)^2 \vec{v}_1 \cdot \vec{v}_2 \vec{v}_2 \cdot \vec{v}_2 + 3 \vec{S}_1 \cdot \vec{S}_1 \vec{v}_1 \cdot \vec{v}_2 \vec{v}_2 \cdot \vec{v}_2 \Big) \Big) m_2^2 C_{\text{ES}^2_1} \} \end{aligned}$$

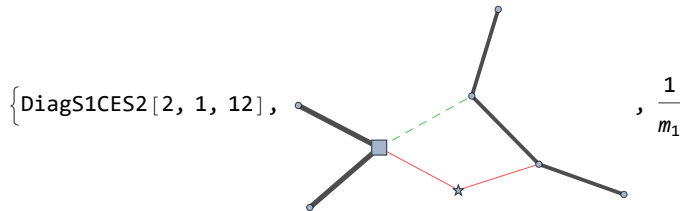

$$\begin{aligned}
G^2 \left( \frac{1}{\kappa^4} \right. & \left( 60 \vec{S}_1 \cdot \vec{S}_1 (\hat{n} \cdot \vec{v}_2)^4 - 168 \hat{n} \cdot \vec{v}_1 \vec{S}_1 \cdot \vec{S}_1 (\hat{n} \cdot \vec{v}_2)^3 + 3 \hat{n} \cdot \vec{S}_1 \vec{S}_1 \cdot \vec{v}_1 (\hat{n} \cdot \vec{v}_2)^3 - 66 \hat{n} \cdot \vec{S}_1 \vec{S}_1 \cdot \vec{v}_2 (\hat{n} \cdot \vec{v}_2)^3 + \right. \\
& \left( \vec{S}_1 \cdot \vec{v}_1 \right)^2 (\hat{n} \cdot \vec{v}_2)^2 + 35 \left( \vec{S}_1 \cdot \vec{v}_2 \right)^2 (\hat{n} \cdot \vec{v}_2)^2 + 84 (\hat{n} \cdot \vec{v}_1)^2 \vec{S}_1 \cdot \vec{S}_1 (\hat{n} \cdot \vec{v}_2)^2 - 6 \hat{n} \cdot \vec{S}_1 \hat{n} \cdot \vec{v}_1 \vec{S}_1 \cdot \vec{v}_1 (\hat{n} \cdot \vec{v}_2)^2 + \\
& 183 \hat{n} \cdot \vec{S}_1 \hat{n} \cdot \vec{v}_1 \vec{S}_1 \cdot \vec{v}_2 (\hat{n} \cdot \vec{v}_2)^2 - 29 \vec{S}_1 \cdot \vec{v}_1 \vec{S}_1 \cdot \vec{v}_2 (\hat{n} \cdot \vec{v}_2)^2 - 14 \vec{S}_1 \cdot \vec{S}_1 \vec{v}_1 \cdot \vec{v}_1 (\hat{n} \cdot \vec{v}_2)^2 - \\
& 66 (\hat{n} \cdot \vec{S}_1)^2 \vec{v}_1 \cdot \vec{v}_2 (\hat{n} \cdot \vec{v}_2)^2 + 80 \vec{S}_1 \cdot \vec{S}_1 \vec{v}_1 \cdot \vec{v}_2 (\hat{n} \cdot \vec{v}_2)^2 - 45 \vec{S}_1 \cdot \vec{S}_1 \vec{v}_2 \cdot \vec{v}_2 (\hat{n} \cdot \vec{v}_2)^2 - \\
& 71 \hat{n} \cdot \vec{v}_1 \left( \vec{S}_1 \cdot \vec{v}_2 \right)^2 \hat{n} \cdot \vec{v}_2 - 90 \hat{n} \cdot \vec{S}_1 (\hat{n} \cdot \vec{v}_1)^2 \vec{S}_1 \cdot \vec{v}_2 \hat{n} \cdot \vec{v}_2 + 27 \hat{n} \cdot \vec{v}_1 \vec{S}_1 \cdot \vec{v}_1 \vec{S}_1 \cdot \vec{v}_2 \hat{n} \cdot \vec{v}_2 + \\
& 15 \hat{n} \cdot \vec{S}_1 \vec{S}_1 \cdot \vec{v}_2 \vec{v}_1 \cdot \vec{v}_1 \hat{n} \cdot \vec{v}_2 + 108 (\hat{n} \cdot \vec{S}_1)^2 \hat{n} \cdot \vec{v}_1 \vec{v}_1 \cdot \vec{v}_2 \hat{n} \cdot \vec{v}_2 - 48 \hat{n} \cdot \vec{v}_1 \vec{S}_1 \cdot \vec{S}_1 \vec{v}_1 \cdot \vec{v}_2 \hat{n} \cdot \vec{v}_2 - \\
& 34 \hat{n} \cdot \vec{S}_1 \vec{S}_1 \cdot \vec{v}_1 \vec{v}_1 \cdot \vec{v}_2 \hat{n} \cdot \vec{v}_2 - 11 \hat{n} \cdot \vec{S}_1 \vec{S}_1 \cdot \vec{v}_2 \vec{v}_1 \cdot \vec{v}_2 \hat{n} \cdot \vec{v}_2 + 72 \hat{n} \cdot \vec{v}_1 \vec{S}_1 \cdot \vec{S}_1 \vec{v}_2 \cdot \vec{v}_2 \hat{n} \cdot \vec{v}_2 - \\
& 3 \hat{n} \cdot \vec{S}_1 \vec{S}_1 \cdot \vec{v}_1 \vec{v}_2 \cdot \vec{v}_2 \hat{n} \cdot \vec{v}_2 + 18 \hat{n} \cdot \vec{S}_1 \vec{S}_1 \cdot \vec{v}_2 \vec{v}_2 \cdot \vec{v}_2 \hat{n} \cdot \vec{v}_2 + 24 (\hat{n} \cdot \vec{v}_1)^2 \left( \vec{S}_1 \cdot \vec{v}_2 \right)^2 - \\
& 18 (\hat{n} \cdot \vec{S}_1)^2 (\vec{v}_1 \cdot \vec{v}_2)^2 + 5 \vec{S}_1 \cdot \vec{S}_1 (\vec{v}_1 \cdot \vec{v}_2)^2 + 3 \vec{S}_1 \cdot \vec{S}_1 (\vec{v}_2 \cdot \vec{v}_2)^2 - 6 \left( \vec{S}_1 \cdot \vec{v}_2 \right)^2 \vec{v}_1 \cdot \vec{v}_1 + \\
& 11 \left( \vec{S}_1 \cdot \vec{v}_2 \right)^2 \vec{v}_1 \cdot \vec{v}_2 - 17 \hat{n} \cdot \vec{S}_1 \hat{n} \cdot \vec{v}_1 \vec{S}_1 \cdot \vec{v}_2 \vec{v}_1 \cdot \vec{v}_2 + 5 \vec{S}_1 \cdot \vec{v}_1 \vec{S}_1 \cdot \vec{v}_2 \vec{v}_1 \cdot \vec{v}_2 - \left( \vec{S}_1 \cdot \vec{v}_1 \right)^2 \vec{v}_2 \cdot \vec{v}_2 - \\
& 5 \left( \vec{S}_1 \cdot \vec{v}_2 \right)^2 \vec{v}_2 \cdot \vec{v}_2 - 20 (\hat{n} \cdot \vec{v}_1)^2 \vec{S}_1 \cdot \vec{S}_1 \vec{v}_2 \cdot \vec{v}_2 + 4 \hat{n} \cdot \vec{S}_1 \hat{n} \cdot \vec{v}_1 \vec{S}_1 \cdot \vec{v}_1 \vec{v}_2 \cdot \vec{v}_2 - \\
& 12 \hat{n} \cdot \vec{S}_1 \hat{n} \cdot \vec{v}_1 \vec{S}_1 \cdot \vec{v}_2 \vec{v}_2 \cdot \vec{v}_2 + 3 \vec{S}_1 \cdot \vec{v}_1 \vec{S}_1 \cdot \vec{v}_2 \vec{v}_2 \cdot \vec{v}_2 + 5 \vec{S}_1 \cdot \vec{S}_1 \vec{v}_1 \cdot \vec{v}_1 \vec{v}_2 \cdot \vec{v}_2 - 12 \vec{S}_1 \cdot \vec{S}_1 \vec{v}_1 \cdot \vec{v}_2 \vec{v}_2 \cdot \vec{v}_2 \Big) + \\
& \frac{1}{\kappa^2} \left( 3 \vec{S}_1 \cdot \vec{S}_1 (\hat{n} \cdot \vec{a}_2)^2 - 3 \hat{n} \cdot \vec{S}_1 \vec{S}_1 \cdot \vec{v}_2 \hat{n} \cdot \vec{a}_2 + 20 \hat{n} \cdot \vec{v}_2 \vec{S}_1 \cdot \vec{S}_1 \hat{n} \cdot \vec{a}_2 - 3 \hat{n} \cdot \vec{S}_1 \vec{S}_1 \cdot \vec{a}_2 \hat{n} \cdot \vec{a}_2 - \right. \\
& 3 \hat{n} \cdot \vec{S}_1 \vec{S}_1 \cdot \vec{v}_2 \hat{n} \cdot \vec{a}_2 - 2 \hat{n} \cdot \vec{v}_2 \vec{S}_1^1 \hat{n} \cdot \vec{a}_2 + 2 \left( \vec{S}_1 \cdot \vec{a}_2 \right)^2 - 7 \hat{n} \cdot \vec{S}_1 \hat{n} \cdot \vec{v}_2 \vec{S}_1 \cdot \vec{a}_2 - 7 \hat{n} \cdot \vec{S}_1 \hat{n} \cdot \vec{v}_2 \vec{S}_1 \cdot \vec{a}_2 - \\
& 7 \hat{n} \cdot \vec{S}_1 \hat{n} \cdot \vec{v}_2 \vec{S}_1 \cdot \vec{a}_2 + 6 \vec{S}_1^1 \cdot \vec{v}_2 \vec{S}_1 \cdot \vec{a}_2 + 5 \hat{n} \cdot \vec{a}_2 \hat{n} \cdot \vec{v}_2 \vec{S}_1 \cdot \vec{S}_1 - 2 \vec{a}_2 \cdot \vec{a}_2 \vec{S}_1 \cdot \vec{S}_1 + \\
& 6 \vec{S}_1^1 \cdot \vec{a}_2 \vec{S}_1 \cdot \vec{v}_2 + 4 \vec{S}_1 \cdot \vec{a}_2 \vec{S}_1 \cdot \vec{v}_2 - 2 \vec{S}_1 \cdot \vec{S}_1 \vec{v}_2 \cdot \vec{a}_2 - 12 \vec{S}_1 \cdot \vec{S}_1 \vec{v}_2 \cdot \vec{a}_2 + 2 \vec{v}_2 \cdot \vec{a}_2 \vec{S}_1^1 \Big) + \\
& \frac{1}{\kappa^3} \left( 40 \vec{S}_1 \cdot \vec{S}_1 (\hat{n} \cdot \vec{v}_2)^3 - 2 \vec{S}_1^1 (\hat{n} \cdot \vec{v}_2)^3 + \hat{n} \cdot \vec{S}_1 \vec{S}_1 \cdot \vec{v}_1 (\hat{n} \cdot \vec{v}_2)^2 - 20 \hat{n} \cdot \vec{S}_1 \vec{S}_1 \cdot \vec{v}_2 (\hat{n} \cdot \vec{v}_2)^2 - \right. \\
& 32 \hat{n} \cdot \vec{v}_1 \vec{S}_1 \cdot \vec{S}_1^1 (\hat{n} \cdot \vec{v}_2)^2 + \hat{n} \cdot \vec{S}_1 \vec{S}_1 \cdot \vec{a}_1 (\hat{n} \cdot \vec{v}_2)^2 - 33 \hat{n} \cdot \vec{S}_1 \vec{S}_1 \cdot \vec{a}_2 (\hat{n} \cdot \vec{v}_2)^2 - 14 \hat{n} \cdot \vec{a}_1 \vec{S}_1 \cdot \vec{S}_1 (\hat{n} \cdot \vec{v}_2)^2 + \\
& 45 \hat{n} \cdot \vec{a}_2 \vec{S}_1 \cdot \vec{S}_1 (\hat{n} \cdot \vec{v}_2)^2 + \hat{n} \cdot \vec{S}_1 \vec{S}_1 \cdot \vec{v}_1 (\hat{n} \cdot \vec{v}_2)^2 - 20 \hat{n} \cdot \vec{S}_1 \vec{S}_1 \cdot \vec{v}_2 (\hat{n} \cdot \vec{v}_2)^2 + 2 \hat{n} \cdot \vec{v}_1 \vec{S}_1^1 (\hat{n} \cdot \vec{v}_2)^2 + \\
& 15 \hat{n} \cdot \vec{S}_1 \hat{n} \cdot \vec{v}_1 \vec{S}_1^1 \cdot \vec{v}_2 \hat{n} \cdot \vec{v}_2 - 18 (\hat{n} \cdot \vec{S}_1)^2 \vec{a}_1 \cdot \vec{v}_2 \hat{n} \cdot \vec{v}_2 + 43 \hat{n} \cdot \vec{S}_1 \hat{n} \cdot \vec{v}_1 \vec{S}_1 \cdot \vec{a}_2 \hat{n} \cdot \vec{v}_2 - 46 \hat{n} \cdot \vec{a}_2 \hat{n} \cdot \vec{v}_1 \vec{S}_1 \cdot \vec{S}_1 \hat{n} \cdot \vec{v}_2 + \\
& 5 \vec{a}_1 \cdot \vec{v}_2 \vec{S}_1 \cdot \vec{S}_1 \hat{n} \cdot \vec{v}_2 + \hat{n} \cdot \vec{a}_2 \hat{n} \cdot \vec{S}_1 \vec{S}_1 \cdot \vec{v}_1 \hat{n} \cdot \vec{v}_2 - 3 \vec{S}_1^1 \cdot \vec{v}_2 \vec{S}_1 \cdot \vec{v}_1 \hat{n} \cdot \vec{v}_2 - 10 \vec{S}_1 \cdot \vec{a}_2 \vec{S}_1 \cdot \vec{v}_1 \hat{n} \cdot \vec{v}_2 + \\
& 15 \hat{n} \cdot \vec{a}_1 \hat{n} \cdot \vec{S}_1 \vec{S}_1 \cdot \vec{v}_2 \hat{n} \cdot \vec{v}_2 - 18 \hat{n} \cdot \vec{a}_2 \hat{n} \cdot \vec{S}_1 \vec{S}_1 \cdot \vec{v}_2 \hat{n} \cdot \vec{v}_2 + 15 \hat{n} \cdot \vec{S}_1 \hat{n} \cdot \vec{v}_1 \vec{S}_1 \cdot \vec{v}_2 \hat{n} \cdot \vec{v}_2 - 3 \vec{S}_1^1 \cdot \vec{v}_1 \vec{S}_1 \cdot \vec{v}_2 \hat{n} \cdot \vec{v}_2 + \\
& 22 \vec{S}_1^1 \cdot \vec{v}_2 \vec{S}_1 \cdot \vec{v}_2 \hat{n} \cdot \vec{v}_2 - 3 \vec{S}_1 \cdot \vec{a}_1 \vec{S}_1 \cdot \vec{v}_2 \hat{n} \cdot \vec{v}_2 + 23 \vec{S}_1 \cdot \vec{a}_2 \vec{S}_1 \cdot \vec{v}_2 \hat{n} \cdot \vec{v}_2 - 18 (\hat{n} \cdot \vec{S}_1)^2 \vec{v}_1 \cdot \vec{a}_2 \hat{n} \cdot \vec{v}_2 + \\
& 13 \vec{S}_1 \cdot \vec{S}_1 \vec{v}_1 \cdot \vec{a}_2 \hat{n} \cdot \vec{v}_2 - 36 \hat{n} \cdot \vec{S}_1 \hat{n} \cdot \vec{S}_1 \vec{v}_1 \cdot \vec{v}_2 \hat{n} \cdot \vec{v}_2 + 10 \vec{S}_1 \cdot$$

$$\begin{aligned}
& 12 \hat{n} \cdot \vec{v}_1 \vec{S}_1^1 \cdot \vec{v}_2 \vec{S}_1^1 \cdot \vec{v}_2 + 8 \hat{n} \cdot \vec{S}_1^1 \vec{a}_1 \cdot \vec{v}_2 \vec{S}_1^1 \cdot \vec{v}_2 - 18 \hat{n} \cdot \vec{v}_1 \vec{S}_1^1 \cdot \vec{a}_2 \vec{S}_1^1 \cdot \vec{v}_2 - 3 \hat{n} \cdot \vec{a}_2 \vec{S}_1^1 \cdot \vec{v}_1 \vec{S}_1^1 \cdot \vec{v}_2 + \\
& 5 \hat{n} \cdot \vec{S}_1^1 \vec{S}_1^1 \cdot \vec{v}_2 \vec{v}_1 \cdot \vec{a}_2 + 8 \hat{n} \cdot \vec{S}_1^1 \vec{S}_1^1 \cdot \vec{v}_2 \vec{v}_1 \cdot \vec{v}_2 - 7 \hat{n} \cdot \vec{S}_1^1 \vec{S}_1^1 \cdot \vec{a}_2 \vec{v}_1 \cdot \vec{v}_2 + 8 \hat{n} \cdot \vec{a}_2 \vec{S}_1^1 \cdot \vec{S}_1^1 \vec{v}_1 \cdot \vec{v}_2 + \\
& 8 \hat{n} \cdot \vec{S}_1^1 \vec{S}_1^1 \cdot \vec{v}_2 \vec{v}_1 \cdot \vec{v}_2 + 13 \hat{n} \cdot \vec{v}_1 \vec{S}_1^1 \cdot \vec{S}_1^1 \vec{v}_2 \cdot \vec{a}_2 - \hat{n} \cdot \vec{S}_1^1 \vec{S}_1^1 \cdot \vec{v}_1 \vec{v}_2 \cdot \vec{a}_2 - \hat{n} \cdot \vec{S}_1^1 \vec{S}_1^1 \cdot \vec{v}_1 \vec{v}_2 \cdot \vec{v}_2 + 3 \hat{n} \cdot \vec{S}_1^1 \vec{S}_1^1 \cdot \vec{v}_2 \vec{v}_2 \cdot \vec{v}_2 + \\
& 14 \hat{n} \cdot \vec{v}_1 \vec{S}_1^1 \cdot \vec{S}_1^1 \vec{v}_2 \cdot \vec{v}_2 - \hat{n} \cdot \vec{S}_1^1 \vec{S}_1^1 \cdot \vec{a}_1 \vec{v}_2 \cdot \vec{v}_2 + 3 \hat{n} \cdot \vec{S}_1^1 \vec{S}_1^1 \cdot \vec{a}_2 \vec{v}_2 \cdot \vec{v}_2 + 5 \hat{n} \cdot \vec{a}_1 \vec{S}_1^1 \cdot \vec{S}_1^1 \vec{v}_2 \cdot \vec{v}_2 - \\
& 6 \hat{n} \cdot \vec{a}_2 \vec{S}_1^1 \cdot \vec{S}_1^1 \vec{v}_2 \cdot \vec{v}_2 - \hat{n} \cdot \vec{S}_1^1 \vec{S}_1^1 \cdot \vec{v}_1 \vec{v}_2 \cdot \vec{v}_2 + 3 \hat{n} \cdot \vec{S}_1^1 \vec{S}_1^1 \cdot \vec{v}_2 \vec{v}_2 \cdot \vec{v}_2 - 2 \hat{n} \cdot \vec{v}_1 \vec{v}_2 \cdot \vec{v}_2 \vec{S}_1^1 \Big) \Big) m_2^2 C_{ES^2 1} \Big\}
\end{aligned}$$

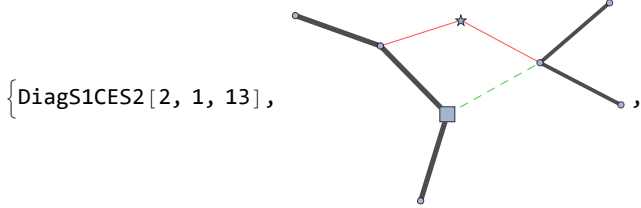

$$\begin{aligned}
& G^2 \left( \frac{1}{r^2} \left( 2 \hat{n} \cdot \vec{v}_1 \hat{n} \cdot \vec{v}_2 \vec{S}_1^1 \cdot \vec{S}_1^1 - \hat{n} \cdot \vec{S}_1^1 \hat{n} \cdot \vec{v}_1 \vec{S}_1^1 \cdot \vec{a}_2 - 2 \hat{n} \cdot \vec{S}_1^1 \hat{n} \cdot \vec{v}_1 \vec{S}_1^1 \cdot \vec{v}_2 - \hat{n} \cdot \vec{S}_1^1 \hat{n} \cdot \vec{v}_1 \vec{S}_1^1 \cdot \vec{v}_2 + \right. \right. \\
& \left. \left. 2 \hat{n} \cdot \vec{a}_2 \hat{n} \cdot \vec{v}_1 \vec{S}_1^1 \cdot \vec{S}_1^1 + 2 \hat{n} \cdot \vec{v}_1 \hat{n} \cdot \vec{v}_2 \vec{S}_1^1 \cdot \vec{S}_1^1 - \hat{n} \cdot \vec{S}_1^1 \hat{n} \cdot \vec{v}_1 \vec{S}_1^1 \cdot \vec{a}_2 - \hat{n} \cdot \vec{S}_1^1 \hat{n} \cdot \vec{v}_1 \vec{S}_1^1 \cdot \vec{v}_2 \right) + \frac{1}{r^4} \right. \\
& \left( -3 (\vec{v}_1 \cdot \vec{v}_2)^2 (\hat{n} \cdot \vec{S}_1^1)^2 - 15 (\hat{n} \cdot \vec{v}_1)^2 \vec{v}_1 \cdot \vec{v}_2 (\hat{n} \cdot \vec{S}_1^1)^2 + 18 \hat{n} \cdot \vec{v}_1 \hat{n} \cdot \vec{v}_2 \vec{v}_1 \cdot \vec{v}_2 (\hat{n} \cdot \vec{S}_1^1)^2 + 6 \hat{n} \cdot \vec{v}_1 \vec{S}_1^1 \cdot \vec{v}_1 \vec{v}_1 \cdot \vec{v}_2 \right. \\
& \left. \hat{n} \cdot \vec{S}_1^1 - 6 \hat{n} \cdot \vec{v}_1 \vec{S}_1^1 \cdot \vec{v}_2 \vec{v}_1 \cdot \vec{v}_2 \hat{n} \cdot \vec{S}_1^1 + \vec{S}_1^1 \cdot \vec{S}_1^1 (\vec{v}_1 \cdot \vec{v}_2)^2 + 3 (\hat{n} \cdot \vec{v}_1)^2 \vec{S}_1^1 \cdot \vec{S}_1^1 \vec{v}_1 \cdot \vec{v}_2 - 4 \hat{n} \cdot \vec{v}_1 \hat{n} \cdot \vec{v}_2 \vec{S}_1^1 \cdot \vec{S}_1^1 \vec{v}_1 \cdot \vec{v}_2 \right) + \\
& \left. \frac{1}{r^3} \left( 3 \hat{n} \cdot \vec{v}_1 \vec{a}_1 \cdot \vec{v}_2 (\hat{n} \cdot \vec{S}_1^1)^2 + 3 \hat{n} \cdot \vec{v}_1 \vec{v}_1 \cdot \vec{a}_2 (\hat{n} \cdot \vec{S}_1^1)^2 + 3 (\hat{n} \cdot \vec{v}_1)^2 \vec{S}_1^1 \cdot \vec{v}_2 \hat{n} \cdot \vec{S}_1^1 - 4 \hat{n} \cdot \vec{v}_1 \hat{n} \cdot \vec{v}_2 \vec{S}_1^1 \cdot \vec{v}_2 \hat{n} \cdot \vec{S}_1^1 + \right. \right. \\
& \left. \left. 6 \hat{n} \cdot \vec{S}_1^1 \hat{n} \cdot \vec{v}_1 \vec{v}_1 \cdot \vec{v}_2 \hat{n} \cdot \vec{S}_1^1 + \vec{S}_1^1 \cdot \vec{v}_2 \vec{v}_1 \cdot \vec{v}_2 \hat{n} \cdot \vec{S}_1^1 + 8 \hat{n} \cdot \vec{v}_1 (\hat{n} \cdot \vec{v}_2)^2 \vec{S}_1^1 \cdot \vec{S}_1^1 - \right. \right. \\
& \left. \left. 6 (\hat{n} \cdot \vec{v}_1)^2 \hat{n} \cdot \vec{v}_2 \vec{S}_1^1 \cdot \vec{S}_1^1 - \hat{n} \cdot \vec{v}_1 \vec{a}_1 \cdot \vec{v}_2 \vec{S}_1^1 \cdot \vec{S}_1^1 - \hat{n} \cdot \vec{v}_1 \vec{S}_1^1 \cdot \vec{v}_2 \vec{S}_1^1 \cdot \vec{v}_1 + 3 \hat{n} \cdot \vec{S}_1^1 (\hat{n} \cdot \vec{v}_1)^2 \vec{S}_1^1 \cdot \vec{v}_2 - \right. \right. \\
& \left. \left. 4 \hat{n} \cdot \vec{S}_1^1 \hat{n} \cdot \vec{v}_1 \hat{n} \cdot \vec{v}_2 \vec{S}_1^1 \cdot \vec{v}_2 - \hat{n} \cdot \vec{v}_1 \vec{S}_1^1 \cdot \vec{v}_1 \vec{S}_1^1 \cdot \vec{v}_2 + 2 \hat{n} \cdot \vec{v}_1 \vec{S}_1^1 \cdot \vec{v}_2 \vec{S}_1^1 \cdot \vec{v}_2 - \hat{n} \cdot \vec{v}_1 \vec{S}_1^1 \cdot \vec{S}_1^1 \vec{v}_1 \cdot \vec{a}_2 - \right. \right. \\
& \left. \left. 2 \hat{n} \cdot \vec{v}_2 \vec{S}_1^1 \cdot \vec{S}_1^1 \vec{v}_1 \cdot \vec{v}_2 + \hat{n} \cdot \vec{S}_1^1 \vec{S}_1^1 \cdot \vec{v}_2 \vec{v}_1 \cdot \vec{v}_2 - 2 \hat{n} \cdot \vec{v}_1 \vec{S}_1^1 \cdot \vec{S}_1^1 \vec{v}_2 \cdot \vec{v}_2 \right) \right) m_2 C_{ES^2 1} \Big\}
\end{aligned}$$

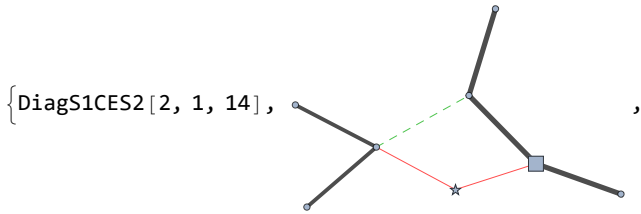

$$\begin{aligned}
& G^2 m_2 C_{ES^2 1} \left( \frac{1}{r^3} \left( 3 \vec{a}_1 \cdot \vec{v}_2 (\hat{n} \cdot \vec{S}_1^1)^2 \hat{n} \cdot \vec{v}_1 + 3 \vec{v}_1 \cdot \vec{a}_2 (\hat{n} \cdot \vec{S}_1^1)^2 \hat{n} \cdot \vec{v}_1 - 2 \vec{a}_1 \cdot \vec{v}_2 \hat{n} \cdot \vec{S}_1^1 \vec{S}_1^1 \cdot \vec{v}_1 - 2 \vec{v}_1 \cdot \vec{a}_2 \hat{n} \cdot \vec{S}_1^1 \vec{S}_1^1 \cdot \vec{v}_1 + \right. \right. \\
& \left. \left. \vec{S}_1^1 \cdot \vec{S}_1^1 \vec{a}_1 \cdot \vec{v}_2 \hat{n} \cdot \vec{v}_1 + \vec{S}_1^1 \cdot \vec{S}_1^1 \vec{v}_1 \cdot \vec{a}_2 \hat{n} \cdot \vec{v}_1 + 2 \vec{v}_1 \cdot \vec{v}_2 \hat{n} \cdot \vec{S}_1^1 \hat{n} \cdot \vec{S}_1^1 \hat{n} \cdot \vec{v}_1 - 8 \vec{v}_1 \cdot \vec{v}_2 \hat{n} \cdot \vec{S}_1^1 \hat{n} \cdot \vec{S}_1^1 \hat{n} \cdot \vec{v}_2 + \right. \right. \\
& \left. \left. 2 \vec{v}_1 \cdot \vec{v}_2 \hat{n} \cdot \vec{S}_1^1 \vec{S}_1^1 \cdot \vec{v}_2 + 2 \vec{S}_1^1 \cdot \vec{S}_1^1 \vec{v}_1 \cdot \vec{v}_2 \hat{n} \cdot \vec{v}_1 - 4 \vec{S}_1^1 \cdot \vec{S}_1^1 \vec{v}_1 \cdot \vec{v}_2 \hat{n} \cdot \vec{v}_2 + 2 \vec{v}_1 \cdot \vec{v}_2 \hat{n} \cdot \vec{S}_1^1 \vec{S}_1^1 \cdot \vec{v}_2 \right) + \right. \\
& \left. \frac{-2 \vec{a}_1 \cdot \vec{v}_2 \hat{n} \cdot \vec{S}_1^1 \hat{n} \cdot \vec{S}_1^1 - 2 \vec{v}_1 \cdot \vec{a}_2 \hat{n} \cdot \vec{S}_1^1 \hat{n} \cdot \vec{S}_1^1 - 2 \vec{S}_1^1 \cdot \vec{S}_1^1 \vec{a}_1 \cdot \vec{v}_2 - 2 \vec{S}_1^1 \cdot \vec{S}_1^1 \vec{v}_1 \cdot \vec{a}_2}{r^2} + \frac{1}{r^4} \right. \\
& \left( -3 (\vec{v}_1 \cdot \vec{v}_2)^2 (\hat{n} \cdot \vec{S}_1^1)^2 - 3 \vec{v}_1 \cdot \vec{v}_2 (\hat{n} \cdot \vec{S}_1^1)^2 (\hat{n} \cdot \vec{v}_1)^2 + 18 \vec{v}_1 \cdot \vec{v}_2 (\hat{n} \cdot \vec{S}_1^1)^2 \hat{n} \cdot \vec{v}_1 \hat{n} \cdot \vec{v}_2 + \right. \\
& \left. 2 \vec{v}_1 \cdot \vec{v}_2 \hat{n} \cdot \vec{S}_1^1 \hat{n} \cdot \vec{v}_1 \vec{S}_1^1 \cdot \vec{v}_1 - 8 \vec{v}_1 \cdot \vec{v}_2 \hat{n} \cdot \vec{S}_1^1 \hat{n} \cdot \vec{v}_2 \vec{S}_1^1 \cdot \vec{v}_1 - 6 \vec{v}_1 \cdot \vec{v}_2 \hat{n} \cdot \vec{S}_1^1 \hat{n} \cdot \vec{v}_1 \vec{S}_1^1 \cdot \vec{v}_2 - \right.
\end{aligned}$$

$$\left. \begin{aligned} & \vec{S}_1 \cdot \vec{S}_1 \vec{v}_1 \cdot \vec{v}_2 \left( \hat{n} \cdot \vec{v}_1 \right)^2 + 4 \vec{S}_1 \cdot \vec{S}_1 \vec{v}_1 \cdot \vec{v}_2 \hat{n} \cdot \vec{v}_1 \hat{n} \cdot \vec{v}_2 - \vec{S}_1 \cdot \vec{S}_1 \left( \vec{v}_1 \cdot \vec{v}_2 \right)^2 + 2 \vec{v}_1 \cdot \vec{v}_2 \vec{S}_1 \cdot \vec{v}_1 \vec{S}_1 \cdot \vec{v}_2 \end{aligned} \right\}$$

$\{\text{DiagS1CES2}[2, 1, 15], \frac{1}{m_1}\}$

$$\begin{aligned}
& \vec{v}_1 \cdot \vec{v}_2 \frac{1}{2} \hat{n} \cdot \vec{v}_2 - \frac{3}{4} \hat{n} \cdot \vec{a}_1 (\vec{S}_1 \cdot \vec{v}_2)^2 - \frac{3}{4} \hat{n} \cdot \vec{a}_2 (\vec{S}_1 \cdot \vec{v}_2)^2 + 4 \hat{n} \cdot \vec{a}_2 (\hat{n} \cdot \vec{v}_1)^2 \vec{S}_1 \cdot \vec{S}_1 - 6 \hat{n} \cdot \vec{a}_2 \hat{n} \cdot \vec{S}_1 \hat{n} \cdot \vec{v}_1 \vec{S}_1 \cdot \vec{v}_2 - \\
& 3 \hat{n} \cdot \vec{v}_1 \vec{S}_1 \cdot \vec{v}_2 \vec{S}_1 \cdot \vec{v}_2 - \frac{3}{2} \hat{n} \cdot \vec{S}_1 \vec{a}_1 \cdot \vec{v}_2 \vec{S}_1 \cdot \vec{v}_2 + \frac{3}{2} \hat{n} \cdot \vec{v}_1 \vec{S}_1 \cdot \vec{a}_2 \vec{S}_1 \cdot \vec{v}_2 + \frac{3}{2} \hat{n} \cdot \vec{a}_2 \vec{S}_1 \cdot \vec{v}_1 \vec{S}_1 \cdot \vec{v}_2 - \\
& 2 \hat{n} \cdot \vec{v}_1 \vec{S}_1 \cdot \vec{S}_1 \vec{v}_1 \cdot \vec{a}_2 + \frac{3}{2} \hat{n} \cdot \vec{S}_1 \vec{S}_1 \cdot \vec{v}_2 \vec{v}_1 \cdot \vec{a}_2 - \hat{n} \cdot \vec{a}_2 \vec{S}_1 \cdot \vec{S}_1 \vec{v}_1 \cdot \vec{v}_1 - 3 \hat{n} \cdot \vec{a}_2 (\hat{n} \cdot \vec{S}_1)^2 \vec{v}_1 \cdot \vec{v}_2 - \\
& 3 \hat{n} \cdot \vec{S}_1 \vec{S}_1 \cdot \vec{v}_2 \vec{v}_1 \cdot \vec{v}_2 + \frac{3}{2} \hat{n} \cdot \vec{S}_1 \vec{S}_1 \cdot \vec{a}_2 \vec{v}_1 \cdot \vec{v}_2 + \hat{n} \cdot \vec{a}_2 \vec{S}_1 \cdot \vec{S}_1 \vec{v}_1 \cdot \vec{v}_2 - 3 \hat{n} \cdot \vec{S}_1 \vec{S}_1 \cdot \vec{v}_2 \vec{v}_1 \cdot \vec{v}_2 - \frac{1}{2} \hat{n} \cdot \vec{v}_1 \vec{S}_1 \cdot \vec{S}_1 \vec{v}_2 \cdot \vec{a}_2 + \\
& 3 \hat{n} \cdot \vec{a}_2 (\hat{n} \cdot \vec{S}_1)^2 \vec{v}_2 \cdot \vec{v}_2 - \frac{3}{2} \hat{n} \cdot \vec{S}_1 \vec{S}_1 \cdot \vec{v}_2 \vec{v}_2 \cdot \vec{v}_2 + 3 \hat{n} \cdot \vec{v}_1 \vec{S}_1 \cdot \vec{S}_1 \vec{v}_2 \cdot \vec{v}_2 - \frac{3}{2} \hat{n} \cdot \vec{S}_1 \vec{S}_1 \cdot \vec{a}_2 \vec{v}_2 \cdot \vec{v}_2 + \\
& \frac{5}{4} \hat{n} \cdot \vec{a}_1 \vec{S}_1 \cdot \vec{S}_1 \vec{v}_2 \cdot \vec{v}_2 - \frac{5}{4} \hat{n} \cdot \vec{a}_2 \vec{S}_1 \cdot \vec{S}_1 \vec{v}_2 \cdot \vec{v}_2 - \frac{3}{2} \hat{n} \cdot \vec{S}_1 \vec{S}_1 \cdot \vec{v}_2 \vec{v}_2 \cdot \vec{v}_2 + \hat{n} \cdot \vec{v}_1 \vec{v}_2 \cdot \vec{v}_2 \vec{S}_1^2 + \frac{\hat{n} \cdot \vec{a}_2 \vec{S}_1^2}{2r} + \\
& \frac{1}{r^2} \left( -\frac{3}{2} (\hat{n} \cdot \vec{S}_1)^2 (\hat{n} \cdot \vec{a}_2)^2 + \frac{1}{2} \vec{S}_1 \cdot \vec{S}_1 (\hat{n} \cdot \vec{a}_2)^2 - 6 \hat{n} \cdot \vec{S}_1 \hat{n} \cdot \vec{S}_1 \hat{n} \cdot \vec{v}_2 \hat{n} \cdot \vec{a}_2 + \frac{3}{2} \hat{n} \cdot \vec{S}_1 \vec{S}_1 \cdot \vec{v}_2 \hat{n} \cdot \vec{a}_2 - \right. \\
& 3 \hat{n} \cdot \vec{v}_2 \vec{S}_1 \cdot \vec{S}_1 \hat{n} \cdot \vec{a}_2 + \frac{3}{2} \hat{n} \cdot \vec{S}_1 \vec{S}_1 \cdot \vec{a}_2 \hat{n} \cdot \vec{a}_2 - \hat{n} \cdot \vec{a}_1 \vec{S}_1 \cdot \vec{S}_1 \hat{n} \cdot \vec{a}_2 + \frac{3}{2} \hat{n} \cdot \vec{S}_1 \vec{S}_1 \cdot \vec{v}_2 \hat{n} \cdot \vec{a}_2 - \\
& 2 \hat{n} \cdot \vec{v}_1 \vec{S}_1^2 \hat{n} \cdot \vec{a}_2 + \frac{5}{2} \hat{n} \cdot \vec{v}_2 \vec{S}_1^2 \hat{n} \cdot \vec{a}_2 + 3 \left( \hat{n} \cdot \vec{S}_1 \right)^2 (\hat{n} \cdot \vec{v}_2)^2 + 3 \hat{n} \cdot \vec{S}_1 \hat{n} \cdot \vec{S}_1 (\hat{n} \cdot \vec{v}_2)^2 + \\
& \frac{3}{4} \left( \vec{S}_1 \cdot \vec{v}_2 \right)^2 - \frac{3}{8} (\vec{S}_1 \cdot \vec{a}_2)^2 + \frac{3}{2} (\hat{n} \cdot \vec{v}_2)^2 \vec{S}_1 \cdot \vec{S}_1 + \frac{3}{2} \hat{n} \cdot \vec{S}_1 \hat{n} \cdot \vec{v}_2 \vec{S}_1 \cdot \vec{a}_2 - 3 \hat{n} \cdot \vec{S}_1 \hat{n} \cdot \vec{v}_2 \vec{S}_1 \cdot \vec{v}_2 - \\
& \frac{3}{2} \hat{n} \cdot \vec{S}_1 \hat{n} \cdot \vec{v}_2 \vec{S}_1 \cdot \vec{v}_2 + \frac{3}{2} (\hat{n} \cdot \vec{v}_2)^2 \vec{S}_1 \cdot \vec{S}_1 + \frac{3}{2} \hat{n} \cdot \vec{S}_1 \hat{n} \cdot \vec{v}_2 \vec{S}_1 \cdot \vec{a}_2 - \frac{3}{4} \vec{S}_1 \cdot \vec{v}_2 \vec{S}_1 \cdot \vec{a}_2 + \frac{1}{2} \vec{a}_1 \cdot \vec{a}_2 \vec{S}_1 \cdot \vec{S}_1 + \\
& \frac{1}{8} \vec{a}_2 \cdot \vec{a}_2 \vec{S}_1 \cdot \vec{S}_1 - \frac{3}{2} \hat{n} \cdot \vec{S}_1 \hat{n} \cdot \vec{v}_2 \vec{S}_1 \cdot \vec{v}_2 - \frac{3}{4} \vec{S}_1 \cdot \vec{a}_2 \vec{S}_1 \cdot \vec{v}_2 + \frac{3}{4} \vec{S}_1 \cdot \vec{v}_2 \vec{S}_1 \cdot \vec{v}_2 + \frac{3}{2} \vec{S}_1 \cdot \vec{S}_1 \vec{v}_2 \cdot \vec{a}_2 - \\
& \left. \frac{3}{4} \vec{S}_1 \cdot \vec{S}_1 \vec{v}_2 \cdot \vec{v}_2 - \frac{3}{4} \vec{S}_1 \cdot \vec{S}_1 \vec{v}_2 \cdot \vec{v}_2 + \vec{v}_1 \cdot \vec{a}_2 \vec{S}_1^2 - \frac{1}{2} \vec{v}_2 \cdot \vec{a}_2 \vec{S}_1^2 - \frac{1}{4} (\hat{n} \cdot \vec{v}_2)^2 \vec{S}_1^2 - \frac{1}{4} \vec{v}_2 \cdot \vec{v}_2 \vec{S}_1^2 \right) \Bigg\} m_2^2 C_{ES^2 1} \}
\end{aligned}$$

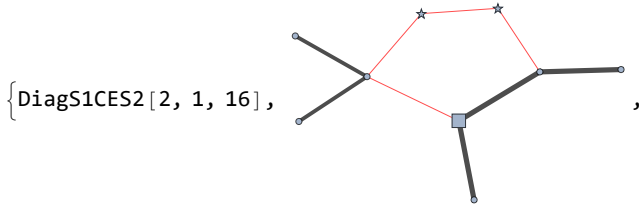

$$\begin{aligned}
& G^2 \left( \frac{\frac{3}{8} \hat{n} \cdot \vec{a}_1 (\hat{n} \cdot \vec{S}_1)^2 + \frac{3}{8} \hat{n} \cdot \vec{S}_1 \hat{n} \cdot \vec{a}_1 \hat{n} \cdot \vec{S}_1 - \frac{1}{8} \hat{n} \cdot \vec{a}_1 \vec{S}_1 \cdot \vec{S}_1 - \frac{1}{8} \hat{n} \cdot \vec{a}_1 \vec{S}_1 \cdot \vec{S}_1}{r} + \frac{1}{r^2} \right. \\
& \left( \frac{3}{8} (\hat{n} \cdot \vec{v}_1)^2 (\hat{n} \cdot \vec{S}_1)^2 + \frac{3}{8} \vec{v}_1 \cdot \vec{v}_1 (\hat{n} \cdot \vec{S}_1)^2 - \frac{15}{4} \hat{n} \cdot \vec{a}_1 \hat{n} \cdot \vec{S}_1 \hat{n} \cdot \vec{v}_1 \hat{n} \cdot \vec{S}_1 + 3 \hat{n} \cdot \vec{a}_1 \hat{n} \cdot \vec{S}_1 \hat{n} \cdot \vec{v}_2 \hat{n} \cdot \vec{S}_1 - \right. \\
& \frac{3}{4} \hat{n} \cdot \vec{S}_1 \vec{a}_1 \cdot \vec{v}_2 \hat{n} \cdot \vec{S}_1 + \frac{3}{4} \hat{n} \cdot \vec{a}_1 \vec{S}_1 \cdot \vec{v}_1 \hat{n} \cdot \vec{S}_1 - \frac{3}{4} \hat{n} \cdot \vec{a}_1 \vec{S}_1 \cdot \vec{v}_2 \hat{n} \cdot \vec{S}_1 - \frac{15}{16} (\hat{n} \cdot \vec{a}_1)^2 (\hat{n} \cdot \vec{S}_1)^2 + \\
& \frac{3}{4} \hat{n} \cdot \vec{a}_1 \hat{n} \cdot \vec{a}_2 (\hat{n} \cdot \vec{S}_1)^2 + \frac{3}{8} \hat{n} \cdot \vec{S}_1 \hat{n} \cdot \vec{S}_1 (\hat{n} \cdot \vec{v}_1)^2 - \frac{1}{8} (\hat{n} \cdot \vec{v}_1)^2 \vec{S}_1 \cdot \vec{S}_1 + \frac{3}{4} \hat{n} \cdot \vec{a}_1 \hat{n} \cdot \vec{S}_1 \vec{S}_1 \cdot \vec{v}_1 - \\
& \frac{3}{4} \hat{n} \cdot \vec{a}_1 \hat{n} \cdot \vec{S}_1 \vec{S}_1 \cdot \vec{v}_2 - \frac{3}{16} (\hat{n} \cdot \vec{S}_1)^2 \vec{a}_1 \cdot \vec{a}_2 + \frac{3}{4} \hat{n} \cdot \vec{a}_1 \hat{n} \cdot \vec{v}_1 \vec{S}_1 \cdot \vec{S}_1 - \frac{1}{2} \hat{n} \cdot \vec{a}_1 \hat{n} \cdot \vec{v}_2 \vec{S}_1 \cdot \vec{S}_1 + \\
& \frac{1}{4} \vec{a}_1 \cdot \vec{v}_2 \vec{S}_1 \cdot \vec{S}_1 - \frac{1}{8} (\hat{n} \cdot \vec{v}_1)^2 \vec{S}_1 \cdot \vec{S}_1 + \frac{3}{8} \hat{n} \cdot \vec{a}_1 \hat{n} \cdot \vec{S}_1 \vec{S}_1 \cdot \vec{a}_1 - \frac{3}{8} \hat{n} \cdot \vec{a}_1 \hat{n} \cdot \vec{S}_1 \vec{S}_1 \cdot \vec{a}_2 + \frac{3}{16} (\hat{n} \cdot \vec{a}_1)^2 \vec{S}_1 \cdot \vec{S}_1 - \\
& \left. \frac{1}{8} \hat{n} \cdot \vec{a}_1 \hat{n} \cdot \vec{a}_2 \vec{S}_1 \cdot \vec{S}_1 + \frac{1}{16} \vec{a}_1 \cdot \vec{a}_2 \vec{S}_1 \cdot \vec{S}_1 + \frac{3}{8} \hat{n} \cdot \vec{S}_1 \hat{n} \cdot \vec{S}_1 \vec{v}_1 \cdot \vec{v}_1 - \frac{1}{8} \vec{S}_1 \cdot \vec{S}_1 \vec{v}_1 \cdot \vec{v}_1 - \frac{1}{8} \vec{S}_1 \cdot \vec{S}_1 \vec{v}_1 \cdot \vec{v}_1 \right) + \frac{1}{r^3}
\end{aligned}$$





$$\left. \frac{3}{8} \vec{S_1} \cdot \vec{S_1} \vec{v_1} \cdot \vec{v_1} \vec{v_1} \cdot \vec{v_2} - \frac{3}{4} \left( \hat{n} \cdot \vec{S_1} \right)^2 \vec{v_1} \cdot \vec{v_1} \vec{v_2} \cdot \vec{v_2} + \frac{1}{8} \vec{S_1} \cdot \vec{S_1} \vec{v_1} \cdot \vec{v_1} \vec{v_2} \cdot \vec{v_2} \right) m_2 C_{\text{ES}^2\text{I}} \Bigg\}$$

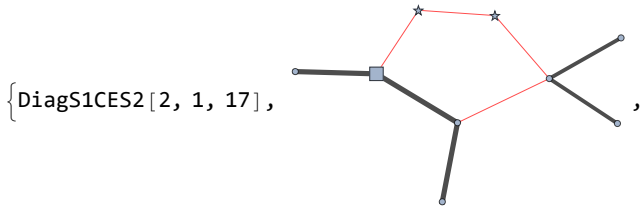

[illegible]



$$\left\{ \frac{3}{8} \vec{S}_1 \cdot \vec{S}_1 \vec{v}_1 \cdot \vec{v}_1 \vec{v}_1 \cdot \vec{v}_2 - \frac{1}{4} \left( \vec{S}_1 \cdot \vec{v}_1 \right)^2 \vec{v}_2 \cdot \vec{v}_2 + \frac{1}{4} \left( \hat{n} \cdot \vec{S}_1 \right)^2 \vec{v}_1 \cdot \vec{v}_1 \vec{v}_2 \cdot \vec{v}_2 + \frac{3}{8} \vec{S}_1 \cdot \vec{S}_1 \vec{v}_1 \cdot \vec{v}_1 \vec{v}_2 \cdot \vec{v}_2 \right\} m_2 C_{ES^2 1}$$

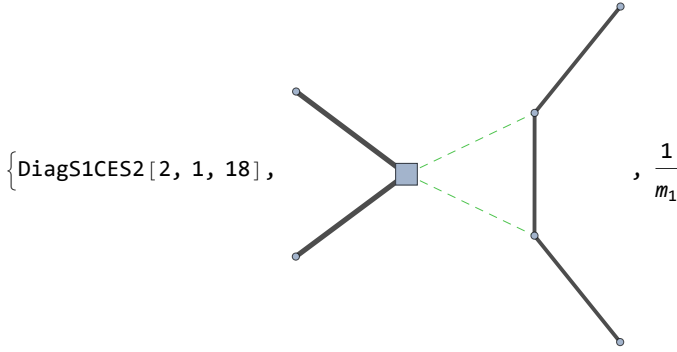

$$G^2 \left( \frac{8 \left( \vec{S}_1 \cdot \vec{a}_2 \right)^2 - 8 \vec{a}_2 \cdot \vec{a}_2 \vec{S}_1 \cdot \vec{S}_1 + 8 \vec{S}_1 \cdot \vec{a}_2 \vec{S}_1 \cdot \vec{v}_2 - 8 \vec{S}_1 \cdot \vec{S}_1 \vec{v}_2 \cdot \vec{a}_2}{r^2} + \frac{1}{r^3} \left( 8 \hat{n} \cdot \vec{a}_2 \left( \vec{S}_1 \cdot \vec{v}_2 \right)^2 - 24 \hat{n} \cdot \vec{v}_1 \vec{S}_1 \cdot \vec{a}_2 \vec{S}_1 \cdot \vec{v}_2 + \right. \right.$$

$$32 \hat{n} \cdot \vec{v}_2 \vec{S}_1 \cdot \vec{a}_2 \vec{S}_1 \cdot \vec{v}_2 + 24 \hat{n} \cdot \vec{S}_1 \vec{v}_1 \cdot \vec{a}_2 \vec{S}_1 \cdot \vec{v}_2 - 24 \hat{n} \cdot \vec{v}_2 \vec{S}_1 \cdot \vec{S}_1 \vec{v}_1 \cdot \vec{a}_2 + 8 \hat{n} \cdot \vec{S}_1 \vec{S}_1 \cdot \vec{a}_2 \vec{v}_1 \cdot \vec{v}_2 -$$

$$8 \hat{n} \cdot \vec{a}_2 \vec{S}_1 \cdot \vec{S}_1 \vec{v}_1 \cdot \vec{v}_2 + 24 \hat{n} \cdot \vec{v}_1 \vec{S}_1 \cdot \vec{S}_1 \vec{v}_2 \cdot \vec{a}_2 - 32 \hat{n} \cdot \vec{v}_2 \vec{S}_1 \cdot \vec{S}_1 \vec{v}_2 \cdot \vec{a}_2 - 8 \hat{n} \cdot \vec{a}_2 \vec{S}_1 \cdot \vec{S}_1 \vec{v}_2 \cdot \vec{v}_2 \left. \right) + \frac{1}{r^4}$$

$$\left( 6 \left( \vec{v}_1 \cdot \vec{v}_2 \right)^2 \left( \hat{n} \cdot \vec{S}_1 \right)^2 + 2 \left( \vec{v}_2 \cdot \vec{v}_2 \right)^2 \left( \hat{n} \cdot \vec{S}_1 \right)^2 + \vec{v}_1 \cdot \vec{v}_1 \vec{v}_2 \cdot \vec{v}_2 \left( \hat{n} \cdot \vec{S}_1 \right)^2 - 2 \hat{n} \cdot \vec{v}_2 \vec{S}_1 \cdot \vec{v}_2 \vec{v}_1 \cdot \vec{v}_1 \hat{n} \cdot \vec{S}_1 + \right.$$

$$2 \hat{n} \cdot \vec{v}_2 \vec{S}_1 \cdot \vec{v}_1 \vec{v}_1 \cdot \vec{v}_2 \hat{n} \cdot \vec{S}_1 - 12 \hat{n} \cdot \vec{v}_1 \vec{S}_1 \cdot \vec{v}_2 \vec{v}_1 \cdot \vec{v}_2 \hat{n} \cdot \vec{S}_1 + 64 \hat{n} \cdot \vec{v}_2 \vec{S}_1 \cdot \vec{v}_2 \vec{v}_1 \cdot \vec{v}_2 \hat{n} \cdot \vec{S}_1 -$$

$$2 \hat{n} \cdot \vec{v}_1 \vec{S}_1 \cdot \vec{v}_1 \vec{v}_2 \cdot \vec{v}_2 \hat{n} \cdot \vec{S}_1 - 4 \hat{n} \cdot \vec{v}_2 \vec{S}_1 \cdot \vec{v}_2 \vec{v}_2 \cdot \vec{v}_2 \hat{n} \cdot \vec{S}_1 + 6 \left( \hat{n} \cdot \vec{v}_1 \right)^2 \left( \vec{S}_1 \cdot \vec{v}_2 \right)^2 + 32 \left( \hat{n} \cdot \vec{v}_2 \right)^2 \left( \vec{S}_1 \cdot \vec{v}_2 \right)^2 -$$

$$40 \hat{n} \cdot \vec{v}_1 \hat{n} \cdot \vec{v}_2 \left( \vec{S}_1 \cdot \vec{v}_2 \right)^2 - 4 \vec{S}_1 \cdot \vec{S}_1 \left( \vec{v}_1 \cdot \vec{v}_2 \right)^2 + 4 \vec{S}_1 \cdot \vec{S}_1 \left( \vec{v}_2 \cdot \vec{v}_2 \right)^2 + 2 \hat{n} \cdot \vec{v}_1 \hat{n} \cdot \vec{v}_2 \vec{S}_1 \cdot \vec{v}_1 \vec{S}_1 \cdot \vec{v}_2 +$$

$$\left( \vec{S}_1 \cdot \vec{v}_2 \right)^2 \vec{v}_1 \cdot \vec{v}_1 + 2 \left( \hat{n} \cdot \vec{v}_2 \right)^2 \vec{S}_1 \cdot \vec{S}_1 \vec{v}_1 \cdot \vec{v}_1 - 8 \left( \vec{S}_1 \cdot \vec{v}_2 \right)^2 \vec{v}_1 \cdot \vec{v}_2 - 64 \left( \hat{n} \cdot \vec{v}_2 \right)^2 \vec{S}_1 \cdot \vec{S}_1 \vec{v}_1 \cdot \vec{v}_2 +$$

$$8 \hat{n} \cdot \vec{v}_1 \hat{n} \cdot \vec{v}_2 \vec{S}_1 \cdot \vec{S}_1 \vec{v}_1 \cdot \vec{v}_2 - 2 \vec{S}_1 \cdot \vec{v}_1 \vec{S}_1 \cdot \vec{v}_2 \vec{v}_1 \cdot \vec{v}_2 - 6 \left( \vec{S}_1 \cdot \vec{v}_2 \right)^2 \vec{v}_2 \cdot \vec{v}_2 - 4 \left( \hat{n} \cdot \vec{v}_1 \right)^2 \vec{S}_1 \cdot \vec{S}_1 \vec{v}_2 \cdot \vec{v}_2 - 28 \left( \hat{n} \cdot \vec{v}_2 \right)^2$$

$$\left. \vec{S}_1 \cdot \vec{S}_1 \vec{v}_2 \cdot \vec{v}_2 + 40 \hat{n} \cdot \vec{v}_1 \hat{n} \cdot \vec{v}_2 \vec{S}_1 \cdot \vec{S}_1 \vec{v}_2 \cdot \vec{v}_2 - 2 \vec{S}_1 \cdot \vec{S}_1 \vec{v}_1 \cdot \vec{v}_1 \vec{v}_2 \cdot \vec{v}_2 + 8 \vec{S}_1 \cdot \vec{S}_1 \vec{v}_1 \cdot \vec{v}_2 \vec{v}_2 \cdot \vec{v}_2 \right) m_2^2 C_{ES^2 1} \Bigg\}$$

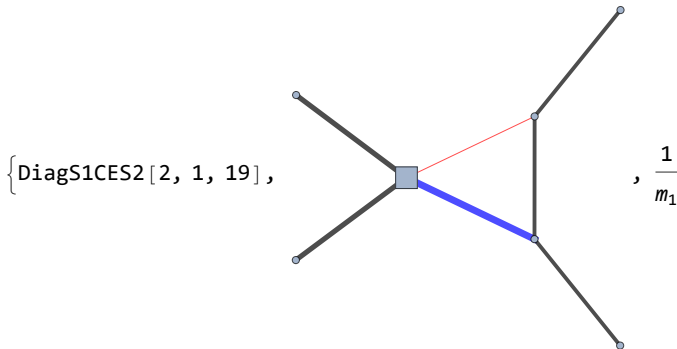

$$G^2 \left( \frac{-2 \left( \vec{S}_1 \cdot \vec{a}_2 \right)^2 - 2 \vec{a}_2 \cdot \vec{a}_2 \vec{S}_1 \cdot \vec{S}_1 - 2 \vec{S}_1 \cdot \vec{a}_2 \vec{S}_1 \cdot \vec{v}_2 - 2 \vec{S}_1 \cdot \vec{S}_1 \vec{v}_2 \cdot \vec{a}_2}{r^2} + \frac{1}{r^3} \right.$$

$$\left( - \left( \hat{n} \cdot \vec{a}_2 \right) \left( \vec{S}_1 \cdot \vec{v}_2 \right)^2 + 12 \hat{n} \cdot \vec{v}_1 \vec{S}_1 \cdot \vec{a}_2 \vec{S}_1 \cdot \vec{v}_2 - 10 \hat{n} \cdot \vec{v}_2 \vec{S}_1 \cdot \vec{a}_2 \vec{S}_1 \cdot \vec{v}_2 + 2 \hat{n} \cdot \vec{a}_2 \vec{S}_1 \cdot \vec{v}_1 \vec{S}_1 \cdot \vec{v}_2 - 6 \hat{n} \cdot \vec{S}_1 \vec{v}_1 \cdot \vec{a}_2 \right.$$

$$\vec{S}_1 \cdot \vec{v}_2 + 2 \hat{n} \cdot \vec{v}_2 \vec{S}_1 \cdot \vec{a}_2 \vec{S}_1 \cdot \vec{v}_1 + 8 \hat{n} \cdot \vec{v}_2 \vec{S}_1 \cdot \vec{S}_1 \vec{v}_1 \cdot \vec{a}_2 - 6 \hat{n} \cdot \vec{S}_1 \vec{S}_1 \cdot \vec{a}_2 \vec{v}_1 \cdot \vec{v}_2 + 8 \hat{n} \cdot \vec{a}_2 \vec{S}_1 \cdot \vec{S}_1 \vec{v}_1 \cdot \vec{v}_2 -$$

$$4 \hat{n} \cdot \vec{v}_1 \vec{S}_1 \cdot \vec{S}_1 \vec{v}_2 \cdot \vec{a}_2 - 10 \hat{n} \cdot \vec{v}_2 \vec{S}_1 \cdot \vec{S}_1 \vec{v}_2 \cdot \vec{a}_2 + 8 \hat{n} \cdot \vec{S}_1 \vec{S}_1 \cdot \vec{v}_1 \vec{v}_2 \cdot \vec{a}_2 - \hat{n} \cdot \vec{a}_2 \vec{S}_1 \cdot \vec{S}_1 \vec{v}_2 \cdot \vec{v}_2 \left. \right) + \frac{1}{r^4}$$

$$\left( -3 \left( \vec{S}_1 \cdot \vec{v}_2 \right)^2 \left( \hat{n} \cdot \vec{v}_1 \right)^2 + \vec{S}_1 \cdot \vec{S}_1 \vec{v}_2 \cdot \vec{v}_2 \left( \hat{n} \cdot \vec{v}_1 \right)^2 + 10 \hat{n} \cdot \vec{v}_2 \left( \vec{S}_1 \cdot \vec{v}_2 \right)^2 \hat{n} \cdot \vec{v}_1 - 12 \hat{n} \cdot \vec{v}_2 \vec{S}_1 \cdot \vec{v}_1 \vec{S}_1 \cdot \vec{v}_2 \hat{n} \cdot \vec{v}_1 -$$

$$\begin{aligned}
& 4 \hat{n} \cdot \vec{v}_2 \vec{S}_1 \cdot \vec{S}_1 \vec{v}_1 \cdot \vec{v}_2 \hat{n} \cdot \vec{v}_1 + 15 \hat{n} \cdot \vec{S}_1 \vec{S}_1 \cdot \vec{v}_2 \vec{v}_1 \cdot \vec{v}_2 \hat{n} \cdot \vec{v}_1 - 2 \hat{n} \cdot \vec{v}_2 \vec{S}_1 \cdot \vec{S}_1 \vec{v}_2 \cdot \vec{v}_2 \hat{n} \cdot \vec{v}_1 - \\
& 6 (\hat{n} \cdot \vec{v}_2)^2 (\vec{S}_1 \cdot \vec{v}_2)^2 - 12 (\hat{n} \cdot \vec{S}_1)^2 (\vec{v}_1 \cdot \vec{v}_2)^2 + 5 \vec{S}_1 \cdot \vec{S}_1 (\vec{v}_1 \cdot \vec{v}_2)^2 - 16 (\hat{n} \cdot \vec{S}_1)^2 (\vec{v}_2 \cdot \vec{v}_2)^2 + \\
& 11 \vec{S}_1 \cdot \vec{S}_1 (\vec{v}_2 \cdot \vec{v}_2)^2 + 8 (\hat{n} \cdot \vec{v}_2)^2 \vec{S}_1 \cdot \vec{v}_1 \vec{S}_1 \cdot \vec{v}_2 - \frac{7}{2} (\vec{S}_1 \cdot \vec{v}_2)^2 \vec{v}_1 \cdot \vec{v}_1 - 12 (\hat{n} \cdot \vec{v}_2)^2 \vec{S}_1 \cdot \vec{S}_1 \vec{v}_1 \cdot \vec{v}_1 + \\
& 12 \hat{n} \cdot \vec{S}_1 \hat{n} \cdot \vec{v}_2 \vec{S}_1 \cdot \vec{v}_2 \vec{v}_1 \cdot \vec{v}_1 + 2 (\vec{S}_1 \cdot \vec{v}_2)^2 \vec{v}_1 \cdot \vec{v}_2 + 12 (\hat{n} \cdot \vec{v}_2)^2 \vec{S}_1 \cdot \vec{S}_1 \vec{v}_1 \cdot \vec{v}_2 - 3 \hat{n} \cdot \vec{S}_1 \hat{n} \cdot \vec{v}_2 \vec{S}_1 \cdot \vec{v}_1 \vec{v}_1 \cdot \vec{v}_2 - \\
& 16 \hat{n} \cdot \vec{S}_1 \hat{n} \cdot \vec{v}_2 \vec{S}_1 \cdot \vec{v}_2 \vec{v}_1 \cdot \vec{v}_2 + \vec{S}_1 \cdot \vec{v}_1 \vec{S}_1 \cdot \vec{v}_2 \vec{v}_1 \cdot \vec{v}_2 - (\vec{S}_1 \cdot \vec{v}_1)^2 \vec{v}_2 \cdot \vec{v}_2 - 5 (\vec{S}_1 \cdot \vec{v}_2)^2 \vec{v}_2 \cdot \vec{v}_2 - \\
& 22 (\hat{n} \cdot \vec{v}_2)^2 \vec{S}_1 \cdot \vec{S}_1 \vec{v}_2 \cdot \vec{v}_2 + 8 \hat{n} \cdot \vec{S}_1 \hat{n} \cdot \vec{v}_2 \vec{S}_1 \cdot \vec{v}_1 \vec{v}_2 \cdot \vec{v}_2 + 16 \hat{n} \cdot \vec{S}_1 \hat{n} \cdot \vec{v}_2 \vec{S}_1 \cdot \vec{v}_2 \vec{v}_2 \cdot \vec{v}_2 - \\
& 4 \vec{S}_1 \cdot \vec{v}_1 \vec{S}_1 \cdot \vec{v}_2 \vec{v}_2 \cdot \vec{v}_2 + \frac{7}{2} \vec{S}_1 \cdot \vec{S}_1 \vec{v}_1 \cdot \vec{v}_1 \vec{v}_2 \cdot \vec{v}_2 - 2 \vec{S}_1 \cdot \vec{S}_1 \vec{v}_1 \cdot \vec{v}_2 \vec{v}_2 \cdot \vec{v}_2 \Big) m_2^2 C_{ES^2_1} \Big\}
\end{aligned}$$

$\{\text{DiagS1CES2}[2, 1, 20],$ 
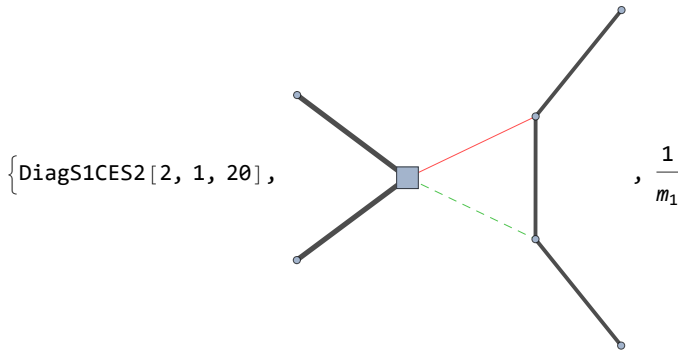
 $, \frac{1}{m_1}$

$$\begin{aligned}
& G^2 \left( \frac{1}{r^3} \left( -2 \hat{n} \cdot \vec{a}_2 (\vec{S}_1 \cdot \vec{v}_1)^2 + 3 \hat{n} \cdot \vec{v}_1 \vec{S}_1 \cdot \vec{a}_2 \vec{S}_1 \cdot \vec{v}_1 - 4 \hat{n} \cdot \vec{a}_2 \vec{S}_1 \cdot \vec{v}_2 \vec{S}_1 \cdot \vec{v}_1 + \right. \right. \\
& 3 \hat{n} \cdot \vec{S}_1 \vec{v}_1 \cdot \vec{a}_2 \vec{S}_1 \cdot \vec{v}_1 - 6 \hat{n} \cdot \vec{v}_1 \vec{S}_1 \cdot \vec{S}_1 \vec{v}_1 \cdot \vec{a}_2 - 3 \hat{n} \cdot \vec{S}_1 \vec{S}_1 \cdot \vec{a}_2 \vec{v}_1 \cdot \vec{v}_1 + 3 \hat{n} \cdot \vec{a}_2 \vec{S}_1 \cdot \vec{S}_1 \vec{v}_1 \cdot \vec{v}_1 + \\
& 28 \hat{n} \cdot \vec{v}_2 \vec{S}_1 \cdot \vec{S}_1 \vec{v}_2 \cdot \vec{a}_2 - 32 \hat{n} \cdot \vec{S}_1 \vec{S}_1 \cdot \vec{v}_2 \vec{v}_2 \cdot \vec{a}_2 - 28 \hat{n} \cdot \vec{S}_1 \vec{S}_1 \cdot \vec{a}_2 \vec{v}_2 \cdot \vec{v}_2 + 20 \hat{n} \cdot \vec{a}_2 \vec{S}_1 \cdot \vec{S}_1 \vec{v}_2 \cdot \vec{v}_2 \Big) + \frac{1}{r^4} \\
& \left( 6 \vec{v}_1 \cdot \vec{v}_1 \vec{v}_1 \cdot \vec{v}_2 (\hat{n} \cdot \vec{S}_1)^2 - 72 \vec{v}_1 \cdot \vec{v}_2 \vec{v}_2 \cdot \vec{v}_2 (\hat{n} \cdot \vec{S}_1)^2 + 3 \hat{n} \cdot \vec{v}_1 \vec{S}_1 \cdot \vec{v}_2 \vec{v}_1 \cdot \vec{v}_1 \hat{n} \cdot \vec{S}_1 - 22 \hat{n} \cdot \vec{v}_2 \vec{S}_1 \cdot \vec{v}_2 \vec{v}_1 \cdot \vec{v}_1 \hat{n} \cdot \vec{S}_1 - \right. \\
& 15 \hat{n} \cdot \vec{v}_1 \vec{S}_1 \cdot \vec{v}_1 \vec{v}_1 \cdot \vec{v}_2 \hat{n} \cdot \vec{S}_1 + 22 \hat{n} \cdot \vec{v}_2 \vec{S}_1 \cdot \vec{v}_1 \vec{v}_1 \cdot \vec{v}_2 \hat{n} \cdot \vec{S}_1 + 4 \hat{n} \cdot \vec{v}_2 \vec{S}_1 \cdot \vec{v}_1 \vec{v}_2 \cdot \vec{v}_2 \hat{n} \cdot \vec{S}_1 + \\
& 60 \hat{n} \cdot \vec{v}_1 \vec{S}_1 \cdot \vec{v}_2 \vec{v}_2 \cdot \vec{v}_2 \hat{n} \cdot \vec{S}_1 - 80 \hat{n} \cdot \vec{v}_2 \vec{S}_1 \cdot \vec{v}_2 \vec{v}_2 \cdot \vec{v}_2 \hat{n} \cdot \vec{S}_1 - 2 (\hat{n} \cdot \vec{v}_2)^2 (\vec{S}_1 \cdot \vec{v}_1)^2 + \hat{n} \cdot \vec{v}_1 \hat{n} \cdot \vec{v}_2 (\vec{S}_1 \cdot \vec{v}_1)^2 + \\
& 2 \vec{S}_1 \cdot \vec{S}_1 (\vec{v}_1 \cdot \vec{v}_2)^2 - 20 \vec{S}_1 \cdot \vec{S}_1 (\vec{v}_2 \cdot \vec{v}_2)^2 - 3 (\hat{n} \cdot \vec{v}_1)^2 \vec{S}_1 \cdot \vec{v}_1 \vec{S}_1 \cdot \vec{v}_2 - 12 (\hat{n} \cdot \vec{v}_2)^2 \vec{S}_1 \cdot \vec{v}_1 \vec{S}_1 \cdot \vec{v}_2 + \\
& 22 \hat{n} \cdot \vec{v}_1 \hat{n} \cdot \vec{v}_2 \vec{S}_1 \cdot \vec{v}_1 \vec{S}_1 \cdot \vec{v}_2 + 5 (\vec{S}_1 \cdot \vec{v}_2)^2 \vec{v}_1 \cdot \vec{v}_1 + 22 (\hat{n} \cdot \vec{v}_2)^2 \vec{S}_1 \cdot \vec{S}_1 \vec{v}_1 \cdot \vec{v}_1 - 2 \hat{n} \cdot \vec{v}_1 \hat{n} \cdot \vec{v}_2 \vec{S}_1 \cdot \vec{S}_1 \vec{v}_1 \cdot \vec{v}_1 + \\
& 6 (\vec{S}_1 \cdot \vec{v}_1)^2 \vec{v}_1 \cdot \vec{v}_2 + 6 (\hat{n} \cdot \vec{v}_1)^2 \vec{S}_1 \cdot \vec{S}_1 \vec{v}_1 \cdot \vec{v}_2 - 16 \hat{n} \cdot \vec{v}_1 \hat{n} \cdot \vec{v}_2 \vec{S}_1 \cdot \vec{S}_1 \vec{v}_1 \cdot \vec{v}_2 - 10 \vec{S}_1 \cdot \vec{v}_1 \vec{S}_1 \cdot \vec{v}_2 \vec{v}_1 \cdot \vec{v}_2 - \\
& 2 \vec{S}_1 \cdot \vec{S}_1 \vec{v}_1 \cdot \vec{v}_1 \vec{v}_1 \cdot \vec{v}_2 + 20 (\vec{S}_1 \cdot \vec{v}_2)^2 \vec{v}_2 \cdot \vec{v}_2 + 72 (\hat{n} \cdot \vec{v}_2)^2 \vec{S}_1 \cdot \vec{S}_1 \vec{v}_2 \cdot \vec{v}_2 - 56 \hat{n} \cdot \vec{v}_1 \hat{n} \cdot \vec{v}_2 \vec{S}_1 \cdot \vec{S}_1 \vec{v}_2 \cdot \vec{v}_2 - \\
& \left. 12 \vec{S}_1 \cdot \vec{v}_1 \vec{S}_1 \cdot \vec{v}_2 \vec{v}_2 \cdot \vec{v}_2 - 5 \vec{S}_1 \cdot \vec{S}_1 \vec{v}_1 \cdot \vec{v}_1 \vec{v}_2 \cdot \vec{v}_2 + 48 \vec{S}_1 \cdot \vec{S}_1 \vec{v}_1 \cdot \vec{v}_2 \vec{v}_2 \cdot \vec{v}_2 \right) m_2^2 C_{ES^2_1} \Big\}
\end{aligned}$$

$\{\text{DiagS1CES2}[2, 1, 21],$ 
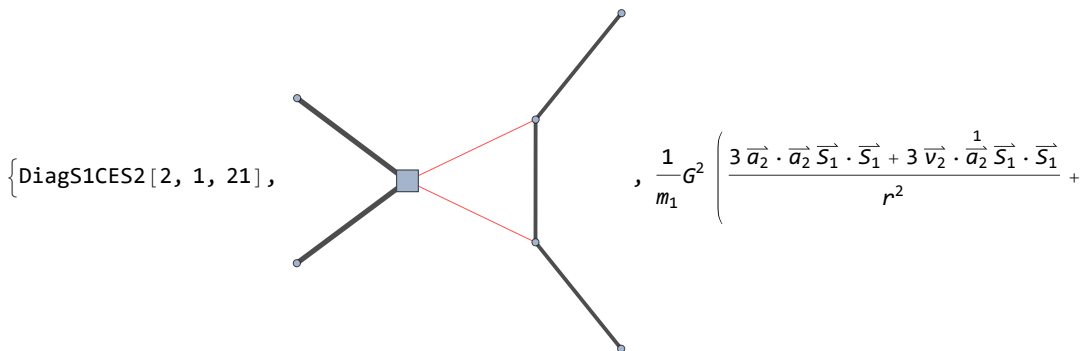
 $, \frac{1}{m_1} G^2 \left( \frac{3 \vec{a}_2 \cdot \vec{a}_2 \vec{S}_1 \cdot \vec{S}_1 + 3 \vec{v}_2 \cdot \vec{a}_2 \vec{S}_1 \cdot \vec{S}_1}{r^2} + \right.$

$$\frac{\frac{5}{2} \hat{n} \cdot \vec{a}_2 (\vec{S}_1 \cdot \vec{v}_1)^2 - 6 \hat{n} \cdot \vec{S}_1 \vec{v}_2 \cdot \vec{a}_2 \vec{S}_1 \cdot \vec{v}_1 - 6 \hat{n} \cdot \vec{v}_1 \vec{S}_1 \cdot \vec{S}_1 \vec{v}_2 \cdot \vec{a}_2 + 18 \hat{n} \cdot \vec{v}_2 \vec{S}_1 \cdot \vec{S}_1 \vec{v}_2 \cdot \vec{a}_2 + 3 \hat{n} \cdot \vec{a}_2 \vec{S}_1 \cdot \vec{S}_1 \vec{v}_2 \cdot \vec{v}_2}{r^3} +$$

$$\begin{aligned}
& \frac{1}{r^4} \left( -\frac{23}{4} (\vec{v}_1 \cdot \vec{v}_1)^2 (\hat{n} \cdot \vec{S}_1)^2 + 24 (\vec{v}_2 \cdot \vec{v}_2)^2 (\hat{n} \cdot \vec{S}_1)^2 - 3 \vec{v}_1 \cdot \vec{v}_1 \vec{v}_2 \cdot \vec{v}_2 (\hat{n} \cdot \vec{S}_1)^2 + \frac{23}{2} \hat{n} \cdot \vec{v}_1 \vec{S}_1 \cdot \vec{v}_1 \vec{v}_1 \cdot \vec{v}_1 \hat{n} \cdot \vec{S}_1 + \right. \\
& 6 \hat{n} \cdot \vec{v}_1 \vec{S}_1 \cdot \vec{v}_1 \vec{v}_2 \cdot \vec{v}_2 \hat{n} \cdot \vec{S}_1 - 12 \hat{n} \cdot \vec{v}_2 \vec{S}_1 \cdot \vec{v}_1 \vec{v}_2 \cdot \vec{v}_2 \hat{n} \cdot \vec{S}_1 - \frac{3}{2} (\hat{n} \cdot \vec{v}_1)^2 (\vec{S}_1 \cdot \vec{v}_1)^2 + 8 (\hat{n} \cdot \vec{v}_2)^2 (\vec{S}_1 \cdot \vec{v}_1)^2 - \\
& 8 \hat{n} \cdot \vec{v}_1 \hat{n} \cdot \vec{v}_2 (\vec{S}_1 \cdot \vec{v}_1)^2 + 3 \vec{S}_1 \cdot \vec{S}_1 (\vec{v}_1 \cdot \vec{v}_1)^2 - 11 \vec{S}_1 \cdot \vec{S}_1 (\vec{v}_2 \cdot \vec{v}_2)^2 - \frac{13}{4} (\vec{S}_1 \cdot \vec{v}_1)^2 \vec{v}_1 \cdot \vec{v}_1 - \\
& 3 (\hat{n} \cdot \vec{v}_1)^2 \vec{S}_1 \cdot \vec{S}_1 \vec{v}_1 \cdot \vec{v}_1 - \frac{1}{2} (\hat{n} \cdot \vec{v}_2)^2 \vec{S}_1 \cdot \vec{S}_1 \vec{v}_1 \cdot \vec{v}_1 - 8 \hat{n} \cdot \vec{v}_1 \hat{n} \cdot \vec{v}_2 \vec{S}_1 \cdot \vec{S}_1 \vec{v}_1 \cdot \vec{v}_1 + \frac{5}{2} (\vec{S}_1 \cdot \vec{v}_1)^2 \vec{v}_1 \cdot \vec{v}_2 + \\
& \frac{5}{2} \vec{S}_1 \cdot \vec{S}_1 \vec{v}_1 \cdot \vec{v}_1 \vec{v}_1 \cdot \vec{v}_2 - 4 (\vec{S}_1 \cdot \vec{v}_1)^2 \vec{v}_2 \cdot \vec{v}_2 + 15 (\hat{n} \cdot \vec{v}_2)^2 \vec{S}_1 \cdot \vec{S}_1 \vec{v}_2 \cdot \vec{v}_2 - 12 \hat{n} \cdot \vec{v}_1 \hat{n} \cdot \vec{v}_2 \vec{S}_1 \cdot \vec{S}_1 \vec{v}_2 \cdot \vec{v}_2 + \\
& \left. 3 \vec{S}_1 \cdot \vec{v}_1 \vec{S}_1 \cdot \vec{v}_2 \vec{v}_2 \cdot \vec{v}_2 + \frac{3}{2} \vec{S}_1 \cdot \vec{S}_1 \vec{v}_1 \cdot \vec{v}_1 \vec{v}_2 \cdot \vec{v}_2 + 3 \vec{S}_1 \cdot \vec{S}_1 \vec{v}_1 \cdot \vec{v}_2 \vec{v}_2 \cdot \vec{v}_2 \right) m_2^2 C_{ES^2_1} \}
\end{aligned}$$

{DiagS1CES2[2, 1, 22],

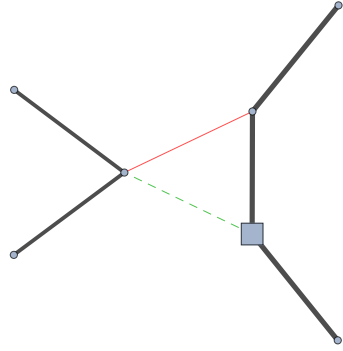

,

$$\begin{aligned}
& G^2 m_2 C_{ES^2_1} \left( \frac{1}{r^3} \left( 2 \vec{S}_1 \cdot \vec{S}_1 \vec{a}_1 \cdot \vec{v}_2 \hat{n} \cdot \vec{v}_1 - 2 \vec{S}_1 \cdot \vec{S}_1 \vec{v}_1 \cdot \vec{a}_1 \hat{n} \cdot \vec{v}_2 + 2 \vec{S}_1 \cdot \vec{S}_1 \vec{v}_1 \cdot \vec{v}_2 \hat{n} \cdot \vec{a}_1 - \vec{a}_1 \cdot \vec{v}_2 \hat{n} \cdot \vec{S}_1 \vec{S}_1 \cdot \vec{v}_1 - \right. \right. \\
& \vec{S}_1 \cdot \vec{a}_1 \hat{n} \cdot \vec{v}_1 \vec{S}_1 \cdot \vec{v}_2 - \hat{n} \cdot \vec{a}_1 \vec{S}_1 \cdot \vec{v}_1 \vec{S}_1 \cdot \vec{v}_2 + 2 \vec{v}_1 \cdot \vec{a}_1 \hat{n} \cdot \vec{S}_1 \vec{S}_1 \cdot \vec{v}_2 - \vec{v}_1 \cdot \vec{v}_2 \vec{S}_1 \cdot \vec{a}_1 \hat{n} \cdot \vec{S}_1 - \hat{n} \cdot \vec{v}_1 \vec{S}_1 \cdot \vec{v}_2 \vec{S}_1 \cdot \vec{v}_1 - \\
& \hat{n} \cdot \vec{v}_1 \vec{S}_1 \cdot \vec{v}_1 \vec{S}_1 \cdot \vec{v}_2 + 4 \vec{v}_1 \cdot \vec{v}_1 \hat{n} \cdot \vec{S}_1 \vec{S}_1 \cdot \vec{v}_2 - 8 \vec{S}_1 \cdot \vec{S}_1 \vec{v}_1 \cdot \vec{v}_1 \hat{n} \cdot \vec{v}_2 + 4 \vec{v}_1 \cdot \vec{v}_1 \hat{n} \cdot \vec{S}_1 \vec{S}_1 \cdot \vec{v}_2 - \vec{v}_1 \cdot \vec{v}_2 \hat{n} \cdot \vec{S}_1 \vec{S}_1 \cdot \vec{v}_1 + \\
& \left. 4 \vec{S}_1 \cdot \vec{S}_1 \vec{v}_1 \cdot \vec{v}_2 \hat{n} \cdot \vec{v}_1 - \vec{v}_1 \cdot \vec{v}_2 \hat{n} \cdot \vec{S}_1 \vec{S}_1 \cdot \vec{v}_1 - 3 \vec{v}_2 \cdot \vec{v}_2 \hat{n} \cdot \vec{S}_1 \vec{S}_1 \cdot \vec{v}_2 + 6 \vec{S}_1 \cdot \vec{S}_1 \vec{v}_2 \cdot \vec{v}_2 \hat{n} \cdot \vec{v}_2 - 3 \vec{v}_2 \cdot \vec{v}_2 \hat{n} \cdot \vec{S}_1 \vec{S}_1 \cdot \vec{v}_2 \right) + \\
& \frac{1}{r^4} \left( -12 \vec{v}_1 \cdot \vec{v}_1 \vec{v}_1 \cdot \vec{v}_2 (\hat{n} \cdot \vec{S}_1)^2 + 9 \vec{v}_1 \cdot \vec{v}_2 \vec{v}_2 \cdot \vec{v}_2 (\hat{n} \cdot \vec{S}_1)^2 + 6 \vec{v}_1 \cdot \vec{v}_2 \hat{n} \cdot \vec{S}_1 \hat{n} \cdot \vec{v}_1 \vec{S}_1 \cdot \vec{v}_1 - \right. \\
& \left. 6 \vec{S}_1 \cdot \vec{S}_1 \vec{v}_1 \cdot \vec{v}_2 (\hat{n} \cdot \vec{v}_1)^2 - 2 \vec{v}_1 \cdot \vec{v}_2 (\vec{S}_1 \cdot \vec{v}_1)^2 + 6 \vec{S}_1 \cdot \vec{S}_1 \vec{v}_1 \cdot \vec{v}_1 \vec{v}_1 \cdot \vec{v}_2 - 3 \vec{S}_1 \cdot \vec{S}_1 \vec{v}_1 \cdot \vec{v}_2 \vec{v}_2 \cdot \vec{v}_2 \right) \}
\end{aligned}$$

{DiagS1CES2[2, 1, 23],

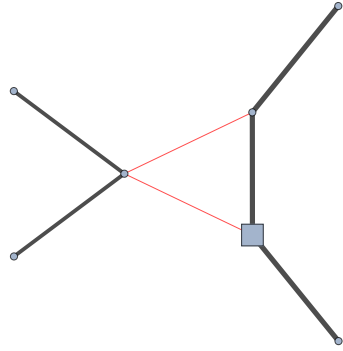

,

$$\begin{aligned}
& G^2 \left( \frac{1}{r^3} \left( \hat{n} \cdot \vec{v}_1 \vec{S}_1 \cdot \vec{v}_1 \vec{S}_1 \cdot \vec{v}_1 + \hat{n} \cdot \vec{v}_1 \vec{S}_1 \cdot \vec{a}_1 \vec{S}_1 \cdot \vec{v}_1 - \frac{3}{2} \hat{n} \cdot \vec{S}_1 \vec{v}_1 \cdot \vec{v}_1 \vec{S}_1 \cdot \vec{v}_1 + \frac{9}{2} \hat{n} \cdot \vec{S}_1 \vec{v}_2 \cdot \vec{v}_2 \vec{S}_1 \cdot \vec{v}_1 - \right. \right. \\
& \hat{n} \cdot \vec{v}_1 \vec{S}_1 \cdot \vec{S}_1 \vec{v}_1 \cdot \vec{a}_1 - \frac{3}{2} \hat{n} \cdot \vec{S}_1 \vec{S}_1 \cdot \vec{v}_1 \vec{v}_1 \cdot \vec{v}_1 + 2 \hat{n} \cdot \vec{v}_1 \vec{S}_1 \cdot \vec{S}_1 \vec{v}_1 \cdot \vec{v}_1 - \frac{3}{2} \hat{n} \cdot \vec{S}_1 \vec{S}_1 \cdot \vec{a}_1 \vec{v}_1 \cdot \vec{v}_1 - \\
& \left. \frac{1}{2} \hat{n} \cdot \vec{a}_1 \vec{S}_1 \cdot \vec{S}_1 \vec{v}_1 \cdot \vec{v}_1 + \frac{9}{2} \hat{n} \cdot \vec{S}_1 \vec{S}_1 \cdot \vec{v}_1 \vec{v}_2 \cdot \vec{v}_2 - 9 \hat{n} \cdot \vec{v}_1 \vec{S}_1 \cdot \vec{S}_1 \vec{v}_2 \cdot \vec{v}_2 + \frac{9}{2} \hat{n} \cdot \vec{S}_1 \vec{S}_1 \cdot \vec{a}_1 \vec{v}_2 \cdot \vec{v}_2 \right) + \frac{1}{r^4}
\end{aligned}$$

$$\left( 6 (\vec{v}_1 \cdot \vec{v}_1)^2 (\hat{n} \cdot \vec{S}_1)^2 - \frac{147}{16} (\vec{v}_2 \cdot \vec{v}_2)^2 (\hat{n} \cdot \vec{S}_1)^2 - \frac{81}{4} \vec{v}_1 \cdot \vec{v}_1 \vec{v}_2 \cdot \vec{v}_2 (\hat{n} \cdot \vec{S}_1)^2 - \frac{39}{8} \hat{n} \cdot \vec{v}_1 \vec{S}_1 \cdot \vec{v}_1 \vec{v}_1 \cdot \vec{v}_1 \hat{n} \cdot \vec{S}_1 + \right. \\ \left. \frac{27}{4} \hat{n} \cdot \vec{v}_1 \vec{S}_1 \cdot \vec{v}_1 \vec{v}_2 \cdot \vec{v}_2 \hat{n} \cdot \vec{S}_1 + \frac{3}{8} (\hat{n} \cdot \vec{v}_1)^2 (\vec{S}_1 \cdot \vec{v}_1)^2 - \frac{7}{2} \vec{S}_1 \cdot \vec{S}_1 (\vec{v}_1 \cdot \vec{v}_1)^2 + \frac{49}{16} \vec{S}_1 \cdot \vec{S}_1 (\vec{v}_2 \cdot \vec{v}_2)^2 + \frac{3}{2} (\vec{S}_1 \cdot \vec{v}_1)^2 \right. \\ \left. \vec{v}_1 \cdot \vec{v}_1 + \frac{9}{2} (\hat{n} \cdot \vec{v}_1)^2 \vec{S}_1 \cdot \vec{S}_1 \vec{v}_1 \cdot \vec{v}_1 - \frac{9}{4} (\vec{S}_1 \cdot \vec{v}_1)^2 \vec{v}_2 \cdot \vec{v}_2 - \frac{27}{4} (\hat{n} \cdot \vec{v}_1)^2 \vec{S}_1 \cdot \vec{S}_1 \vec{v}_2 \cdot \vec{v}_2 + 9 \vec{S}_1 \cdot \vec{S}_1 \vec{v}_1 \cdot \vec{v}_1 \vec{v}_2 \cdot \vec{v}_2 \right) + \\ \left. \frac{1}{r^2} \left( - \left( \frac{1}{\vec{S}_1 \cdot \vec{v}_1} \right)^2 - 2 \vec{S}_1 \cdot \vec{a}_1 \frac{1}{\vec{S}_1 \cdot \vec{v}_1} - (\vec{S}_1 \cdot \vec{a}_1)^2 - 2 \frac{1}{\vec{S}_1 \cdot \vec{a}_1} \vec{S}_1 \cdot \vec{v}_1 - \frac{2}{\vec{S}_1 \cdot \vec{v}_1} \vec{S}_1 \cdot \vec{v}_1 - \vec{S}_1 \cdot \vec{a}_1 \vec{S}_1 \cdot \vec{v}_1 + \right. \right. \\ \left. \left. 4 \vec{S}_1 \cdot \vec{S}_1 \vec{v}_1 \cdot \vec{a}_1 + \frac{1}{\vec{S}_1 \cdot \vec{S}_1} \frac{1}{\vec{v}_1 \cdot \vec{v}_1} + \vec{S}_1 \cdot \vec{S}_1 \frac{2}{\vec{v}_1 \cdot \vec{v}_1} - 2 \vec{v}_1 \cdot \vec{a}_1 \frac{1}{\vec{S}_1^2} - 2 \vec{v}_1 \cdot \vec{v}_1 \frac{2}{\vec{S}_1^2} + \frac{9}{2} \vec{v}_2 \cdot \vec{v}_2 \frac{2}{\vec{S}_1^2} \right) \right) m_2 C_{ES^2 1} \}$$

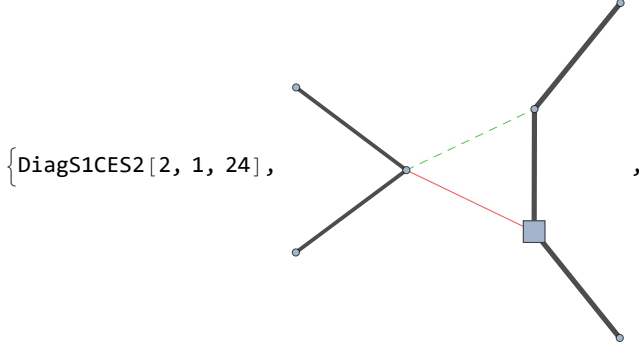

$$G^2 m_2 C_{ES^2 1} \left\{ \frac{4 \vec{v}_1 \cdot \vec{v}_2 \vec{S}_1 \cdot \vec{a}_1 \hat{n} \cdot \vec{S}_1 + 4 \vec{v}_1 \cdot \vec{v}_2 \hat{n} \cdot \vec{S}_1 \frac{1}{\vec{S}_1 \cdot \vec{v}_1} - 8 \vec{S}_1 \cdot \vec{S}_1 \vec{v}_1 \cdot \vec{v}_2 \hat{n} \cdot \vec{v}_1 + 4 \vec{v}_1 \cdot \vec{v}_2 \hat{n} \cdot \frac{1}{\vec{S}_1 \cdot \vec{v}_1} \vec{S}_1 \cdot \vec{v}_1}{r^3} + \right. \\ \left. \frac{1}{r^4} \left( -12 \vec{v}_1 \cdot \vec{v}_1 \vec{v}_1 \cdot \vec{v}_2 (\hat{n} \cdot \vec{S}_1)^2 + 9 \vec{v}_1 \cdot \vec{v}_2 \vec{v}_2 \cdot \vec{v}_2 (\hat{n} \cdot \vec{S}_1)^2 + 6 \vec{v}_1 \cdot \vec{v}_2 \hat{n} \cdot \vec{S}_1 \hat{n} \cdot \vec{v}_1 \vec{S}_1 \cdot \vec{v}_1 - \right. \right. \\ \left. \left. 6 \vec{S}_1 \cdot \vec{S}_1 \vec{v}_1 \cdot \vec{v}_2 (\hat{n} \cdot \vec{v}_1)^2 - 2 \vec{v}_1 \cdot \vec{v}_2 (\vec{S}_1 \cdot \vec{v}_1)^2 + 6 \vec{S}_1 \cdot \vec{S}_1 \vec{v}_1 \cdot \vec{v}_1 \vec{v}_1 \cdot \vec{v}_2 - 3 \vec{S}_1 \cdot \vec{S}_1 \vec{v}_1 \cdot \vec{v}_2 \vec{v}_2 \cdot \vec{v}_2 \right) + \frac{4 \vec{S}_1^2 \vec{v}_1 \cdot \vec{v}_2}{r^2} \right\}$$

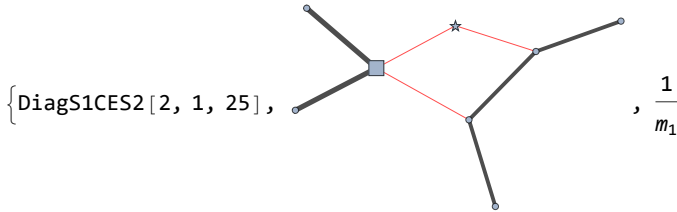

$$G^2 \left\{ \frac{1}{r^4} \left( 15 \vec{S}_1 \cdot \vec{S}_1 (\hat{n} \cdot \vec{v}_2)^4 - 42 \hat{n} \cdot \vec{v}_1 \vec{S}_1 \cdot \vec{S}_1 (\hat{n} \cdot \vec{v}_2)^3 - 12 \hat{n} \cdot \vec{S}_1 \vec{S}_1 \cdot \vec{v}_1 (\hat{n} \cdot \vec{v}_2)^3 - 8 (\vec{S}_1 \cdot \vec{v}_1)^2 (\hat{n} \cdot \vec{v}_2)^2 + \right. \right. \\ 24 (\hat{n} \cdot \vec{v}_1)^2 \vec{S}_1 \cdot \vec{S}_1 (\hat{n} \cdot \vec{v}_2)^2 + 30 \hat{n} \cdot \vec{S}_1 \hat{n} \cdot \vec{v}_1 \vec{S}_1 \cdot \vec{v}_1 (\hat{n} \cdot \vec{v}_2)^2 + 6 \vec{S}_1 \cdot \vec{v}_1 \vec{S}_1 \cdot \vec{v}_2 (\hat{n} \cdot \vec{v}_2)^2 - \\ 3 (\hat{n} \cdot \vec{S}_1)^2 \vec{v}_1 \cdot \vec{v}_1 (\hat{n} \cdot \vec{v}_2)^2 - \frac{3}{2} \vec{S}_1 \cdot \vec{S}_1 \vec{v}_1 \cdot \vec{v}_1 (\hat{n} \cdot \vec{v}_2)^2 + 21 \vec{S}_1 \cdot \vec{S}_1 \vec{v}_1 \cdot \vec{v}_2 (\hat{n} \cdot \vec{v}_2)^2 + 54 (\hat{n} \cdot \vec{S}_1)^2 \vec{v}_2 \cdot \vec{v}_2 \\ (\hat{n} \cdot \vec{v}_2)^2 - 17 \vec{S}_1 \cdot \vec{S}_1 \vec{v}_2 \cdot \vec{v}_2 (\hat{n} \cdot \vec{v}_2)^2 + 8 \hat{n} \cdot \vec{v}_1 (\vec{S}_1 \cdot \vec{v}_1)^2 \hat{n} \cdot \vec{v}_2 - 12 \hat{n} \cdot \vec{S}_1 (\hat{n} \cdot \vec{v}_1)^2 \vec{S}_1 \cdot \vec{v}_1 \hat{n} \cdot \vec{v}_2 - \\ 6 \hat{n} \cdot \vec{v}_1 \vec{S}_1 \cdot \vec{v}_1 \vec{S}_1 \cdot \vec{v}_2 \hat{n} \cdot \vec{v}_2 + 6 (\hat{n} \cdot \vec{S}_1)^2 \hat{n} \cdot \vec{v}_1 \vec{v}_1 \cdot \vec{v}_1 \hat{n} \cdot \vec{v}_2 - 2 \hat{n} \cdot \vec{v}_1 \vec{S}_1 \cdot \vec{S}_1 \vec{v}_1 \cdot \vec{v}_1 \hat{n} \cdot \vec{v}_2 - \\ 2 \hat{n} \cdot \vec{S}_1 \vec{S}_1 \cdot \vec{v}_2 \vec{v}_1 \cdot \vec{v}_1 \hat{n} \cdot \vec{v}_2 - 20 \hat{n} \cdot \vec{v}_1 \vec{S}_1 \cdot \vec{S}_1 \vec{v}_1 \cdot \vec{v}_2 \hat{n} \cdot \vec{v}_2 - 6 \hat{n} \cdot \vec{S}_1 \vec{S}_1 \cdot \vec{v}_1 \vec{v}_1 \cdot \vec{v}_2 \hat{n} \cdot \vec{v}_2 - \\ 108 (\hat{n} \cdot \vec{S}_1)^2 \hat{n} \cdot \vec{v}_1 \vec{v}_2 \cdot \vec{v}_2 \hat{n} \cdot \vec{v}_2 + 20 \hat{n} \cdot \vec{v}_1 \vec{S}_1 \cdot \vec{S}_1 \vec{v}_2 \cdot \vec{v}_2 \hat{n} \cdot \vec{v}_2 + 40 \hat{n} \cdot \vec{S}_1 \vec{S}_1 \cdot \vec{v}_1 \vec{v}_2 \cdot \vec{v}_2 \hat{n} \cdot \vec{v}_2 - \\ 36 \hat{n} \cdot \vec{S}_1 \vec{S}_1 \cdot \vec{v}_2 \vec{v}_2 \cdot \vec{v}_2 \hat{n} \cdot \vec{v}_2 + \frac{7}{2} \vec{S}_1 \cdot \vec{S}_1 (\vec{v}_1 \cdot \vec{v}_2)^2 + \frac{1}{2} \vec{S}_1 \cdot \vec{S}_1 (\vec{v}_2 \cdot \vec{v}_2)^2 - 2 (\hat{n} \cdot \vec{v}_1)^2 \vec{S}_1 \cdot \vec{v}_1 \vec{S}_1 \cdot \vec{v}_2 + \\ \left. \frac{5}{4} (\vec{S}_1 \cdot \vec{v}_2)^2 \vec{v}_1 \cdot \vec{v}_1 + 2 \hat{n} \cdot \vec{S}_1 \hat{n} \cdot \vec{v}_1 \vec{S}_1 \cdot \vec{v}_2 \vec{v}_1 \cdot \vec{v}_1 - (\vec{S}_1 \cdot \vec{v}_1)^2 \vec{v}_1 \cdot \vec{v}_2 + 4 (\hat{n} \cdot \vec{v}_1)^2 \vec{S}_1 \cdot \vec{S}_1 \vec{v}_1 \cdot \vec{v}_2 - \right. \\ \left. \right\}$$

[illegible]

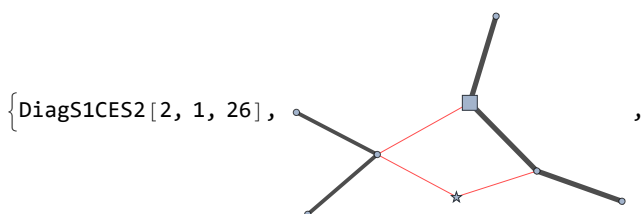



$$\begin{aligned}
G^2 \left( \frac{1}{r^3} \left( \frac{3}{2} \vec{S}_1 \cdot \vec{S}_1 (\hat{n} \cdot \vec{v}_1)^3 - \frac{3}{4} \hat{n} \cdot \vec{S}_1 \vec{S}_1 \cdot \vec{v}_1 (\hat{n} \cdot \vec{v}_1)^2 - 4 \hat{n} \cdot \vec{v}_2 \vec{S}_1 \cdot \vec{S}_1 (\hat{n} \cdot \vec{v}_1)^2 - \frac{3}{4} \hat{n} \cdot \vec{S}_1 \vec{S}_1 \cdot \vec{a}_1 (\hat{n} \cdot \vec{v}_1)^2 - \right. \right. \\
\frac{3}{2} \hat{n} \cdot \vec{a}_1 \vec{S}_1 \cdot \vec{S}_1 (\hat{n} \cdot \vec{v}_1)^2 - \frac{3}{4} \hat{n} \cdot \vec{S}_1 \vec{S}_1 \cdot \vec{v}_1 (\hat{n} \cdot \vec{v}_1)^2 + 2 \hat{n} \cdot \vec{S}_1 \hat{n} \cdot \vec{v}_2 \vec{S}_1 \cdot \vec{v}_1 \hat{n} \cdot \vec{v}_1 + \\
2 \hat{n} \cdot \vec{S}_1 \hat{n} \cdot \vec{v}_2 \vec{S}_1 \cdot \vec{a}_1 \hat{n} \cdot \vec{v}_1 + \frac{3}{4} \hat{n} \cdot \vec{a}_1 \hat{n} \cdot \vec{S}_1 \vec{S}_1 \cdot \vec{v}_1 \hat{n} \cdot \vec{v}_1 + 2 \hat{n} \cdot \vec{S}_1 \hat{n} \cdot \vec{v}_2 \vec{S}_1 \cdot \vec{v}_1 \hat{n} \cdot \vec{v}_1 + \\
\frac{1}{2} \vec{S}_1 \cdot \vec{v}_1 \vec{S}_1 \cdot \vec{v}_1 \hat{n} \cdot \vec{v}_1 - \frac{1}{2} \vec{S}_1 \cdot \vec{v}_2 \vec{S}_1 \cdot \vec{v}_1 \hat{n} \cdot \vec{v}_1 - \frac{1}{2} \vec{S}_1 \cdot \vec{v}_1 \vec{S}_1 \cdot \vec{v}_2 \hat{n} \cdot \vec{v}_1 - \frac{1}{2} \vec{S}_1 \cdot \vec{a}_1 \vec{S}_1 \cdot \vec{v}_2 \hat{n} \cdot \vec{v}_1 + \\
9 (\hat{n} \cdot \vec{S}_1)^2 \vec{v}_1 \cdot \vec{a}_1 \hat{n} \cdot \vec{v}_1 - \vec{S}_1 \cdot \vec{S}_1 \vec{v}_1 \cdot \vec{a}_1 \hat{n} \cdot \vec{v}_1 - \frac{9}{2} \hat{n} \cdot \vec{S}_1 \hat{n} \cdot \vec{S}_1 \vec{v}_1 \cdot \vec{v}_1 \hat{n} \cdot \vec{v}_1 + \vec{S}_1 \cdot \vec{S}_1 \vec{v}_1 \cdot \vec{v}_1 \hat{n} \cdot \vec{v}_1 + \\
2 \vec{S}_1 \cdot \vec{S}_1 \vec{v}_1 \cdot \vec{v}_2 \hat{n} \cdot \vec{v}_1 + \frac{27}{4} (\hat{n} \cdot \vec{S}_1)^2 \vec{v}_2 \cdot \vec{a}_2 \hat{n} \cdot \vec{v}_1 - \frac{9}{4} \vec{S}_1 \cdot \vec{S}_1 \vec{v}_2 \cdot \vec{a}_2 \hat{n} \cdot \vec{v}_1 + \frac{27}{4} \hat{n} \cdot \vec{S}_1 \hat{n} \cdot \vec{S}_1 \vec{v}_2 \cdot \vec{v}_2 \hat{n} \cdot \vec{v}_1 - \\
\frac{9}{4} \vec{S}_1 \cdot \vec{S}_1 \vec{v}_2 \cdot \vec{v}_2 \hat{n} \cdot \vec{v}_1 - 9 (\hat{n} \cdot \vec{S}_1)^2 \hat{n} \cdot \vec{v}_2 \vec{v}_1 \cdot \vec{a}_1 + \frac{3}{2} \hat{n} \cdot \vec{v}_2 \vec{S}_1 \cdot \vec{S}_1 \vec{v}_1 \cdot \vec{a}_1 - \frac{9}{2} \hat{n} \cdot \vec{S}_1 \vec{S}_1 \cdot \vec{v}_1 \vec{v}_1 \cdot \vec{a}_1 + \\
\left. \frac{9}{2} \hat{n} \cdot \vec{S}_1 \vec{S}_1 \cdot \vec{v}_2 \vec{v}_1 \cdot \vec{a}_1 - \frac{1}{2} \hat{n} \cdot \vec{S}_1 \vec{S}_1 \cdot \vec{v}_1 \vec{v}_1 \cdot \vec{v}_2 - \frac{1}{2} \hat{n} \cdot \vec{S}_1 \vec{S}_1 \cdot \vec{a}_1 \vec{v}_1 \cdot \vec{v}_2 - \frac{1}{2} \hat{n} \cdot \vec{S}_1 \vec{S}_1 \cdot \vec{v}_1 \vec{v}_1 \cdot \vec{v}_2 \right) + \frac{1}{r^4} \\
\left( \frac{15}{4} \vec{S}_1 \cdot \vec{S}_1 (\hat{n} \cdot \vec{v}_1)^4 - \frac{9}{2} \hat{n} \cdot \vec{v}_2 \vec{S}_1 \cdot \vec{S}_1 (\hat{n} \cdot \vec{v}_1)^3 - \frac{15}{4} \hat{n} \cdot \vec{S}_1 \vec{S}_1 \cdot \vec{v}_1 (\hat{n} \cdot \vec{v}_1)^3 + \frac{3}{2} (\vec{S}_1 \cdot \vec{v}_1)^2 (\hat{n} \cdot \vec{v}_1)^2 + \right. \\
\frac{9}{2} \hat{n} \cdot \vec{S}_1 \hat{n} \cdot \vec{v}_2 \vec{S}_1 \cdot \vec{v}_1 (\hat{n} \cdot \vec{v}_1)^2 - \frac{3}{4} \vec{S}_1 \cdot \vec{v}_1 \vec{S}_1 \cdot \vec{v}_2 (\hat{n} \cdot \vec{v}_1)^2 + \frac{45}{4} (\hat{n} \cdot \vec{S}_1)^2 \vec{v}_1 \cdot \vec{v}_1 (\hat{n} \cdot \vec{v}_1)^2 - \\
\frac{9}{2} \vec{S}_1 \cdot \vec{S}_1 \vec{v}_1 \cdot \vec{v}_1 (\hat{n} \cdot \vec{v}_1)^2 + \frac{9}{4} \vec{S}_1 \cdot \vec{S}_1 \vec{v}_1 \cdot \vec{v}_2 (\hat{n} \cdot \vec{v}_1)^2 - \frac{135}{8} (\hat{n} \cdot \vec{S}_1)^2 \vec{v}_2 \cdot \vec{v}_2 (\hat{n} \cdot \vec{v}_1)^2 + \\
\frac{27}{8} \vec{S}_1 \cdot \vec{S}_1 \vec{v}_2 \cdot \vec{v}_2 (\hat{n} \cdot \vec{v}_1)^2 - \hat{n} \cdot \vec{v}_2 (\vec{S}_1 \cdot \vec{v}_1)^2 \hat{n} \cdot \vec{v}_1 - \frac{27}{2} (\hat{n} \cdot \vec{S}_1)^2 \hat{n} \cdot \vec{v}_2 \vec{v}_1 \cdot \vec{v}_1 \hat{n} \cdot \vec{v}_1 + \\
4 \hat{n} \cdot \vec{v}_2 \vec{S}_1 \cdot \vec{S}_1 \vec{v}_1 \cdot \vec{v}_1 \hat{n} \cdot \vec{v}_1 - \frac{15}{4} \hat{n} \cdot \vec{S}_1 \vec{S}_1 \cdot \vec{v}_1 \vec{v}_1 \cdot \vec{v}_1 \hat{n} \cdot \vec{v}_1 + \frac{9}{2} \hat{n} \cdot \vec{S}_1 \vec{S}_1 \cdot \vec{v}_2 \vec{v}_1 \cdot \vec{v}_1 \hat{n} \cdot \vec{v}_1 - \\
\frac{3}{2} \hat{n} \cdot \vec{S}_1 \vec{S}_1 \cdot \vec{v}_1 \vec{v}_1 \cdot \vec{v}_2 \hat{n} \cdot \vec{v}_1 + \frac{81}{4} (\hat{n} \cdot \vec{S}_1)^2 \hat{n} \cdot \vec{v}_2 \vec{v}_2 \cdot \vec{v}_2 \hat{n} \cdot \vec{v}_1 - \frac{9}{2} \hat{n} \cdot \vec{v}_2 \vec{S}_1 \cdot \vec{S}_1 \vec{v}_2 \cdot \vec{v}_2 \hat{n} \cdot \vec{v}_1 + \\
\frac{27}{4} \hat{n} \cdot \vec{S}_1 \vec{S}_1 \cdot \vec{v}_1 \vec{v}_2 \cdot \vec{v}_2 \hat{n} \cdot \vec{v}_1 - \frac{27}{4} \hat{n} \cdot \vec{S}_1 \vec{S}_1 \cdot \vec{v}_2 \vec{v}_2 \cdot \vec{v}_2 \hat{n} \cdot \vec{v}_1 + \frac{1}{4} (\vec{S}_1 \cdot \vec{v}_1)^2 \vec{v}_1 \cdot \vec{v}_2 + \\
\frac{9}{4} (\hat{n} \cdot \vec{S}_1)^2 \vec{v}_1 \cdot \vec{v}_1 \vec{v}_1 \cdot \vec{v}_2 - \vec{S}_1 \cdot \vec{S}_1 \vec{v}_1 \cdot \vec{v}_1 \vec{v}_1 \cdot \vec{v}_2 - \frac{27}{8} (\hat{n} \cdot \vec{S}_1)^2 \vec{v}_1 \cdot \vec{v}_2 \vec{v}_2 \cdot \vec{v}_2 + \frac{9}{8} \vec{S}_1 \cdot \vec{S}_1 \vec{v}_1 \cdot \vec{v}_2 \vec{v}_2 \cdot \vec{v}_2 \left. \right) + \\
\frac{1}{r^2} \left( - \left( \frac{1}{\vec{S}_1 \cdot \vec{S}_1} \right) (\hat{n} \cdot \vec{v}_1)^2 - \vec{S}_1 \cdot \vec{S}_1 (\hat{n} \cdot \vec{v}_1)^2 - \frac{1}{2} \vec{S}_1^2 (\hat{n} \cdot \vec{v}_1)^2 + \hat{n} \cdot \vec{S}_1 \vec{S}_1 \cdot \vec{a}_1 \hat{n} \cdot \vec{v}_1 + \hat{n} \cdot \vec{S}_1 \vec{S}_1 \cdot \vec{v}_1 \hat{n} \cdot \vec{v}_1 + \right. \\
\frac{1}{2} \hat{n} \cdot \vec{S}_1 \vec{S}_1 \cdot \vec{v}_1 \hat{n} \cdot \vec{v}_1 + \frac{1}{2} \hat{n} \cdot \vec{S}_1 \vec{S}_1 \cdot \vec{a}_1 \hat{n} \cdot \vec{v}_1 - 2 \hat{n} \cdot \vec{a}_1 \vec{S}_1 \cdot \vec{S}_1 \hat{n} \cdot \vec{v}_1 + \hat{n} \cdot \vec{S}_1 \vec{S}_1 \cdot \vec{a}_1 \hat{n} \cdot \vec{v}_1 + \frac{1}{2} \hat{n} \cdot \vec{S}_1 \vec{S}_1 \cdot \vec{v}_1 \hat{n} \cdot \vec{v}_1 + \\
\left. \frac{1}{2} \hat{n} \cdot \vec{a}_1 \vec{S}_1^2 \hat{n} \cdot \vec{v}_1 + \hat{n} \cdot \vec{v}_2 \vec{S}_1^2 \hat{n} \cdot \vec{v}_1 - \frac{9}{2} \hat{n} \cdot \vec{S}_1 \hat{n} \cdot \vec{S}_1 \vec{v}_1 \cdot \vec{a}_1 + \frac{3}{2} \vec{S}_1 \cdot \vec{S}_1 \vec{v}_1 \cdot \vec{a}_1 - \frac{1}{2} \vec{v}_1 \cdot \vec{v}_2 \vec{S}_1^2 \right) + \frac{\hat{n} \cdot \vec{v}_1 \vec{S}_1^3}{2r} \Bigg\} m_2 C_{ES^2 1} \}
\end{aligned}$$

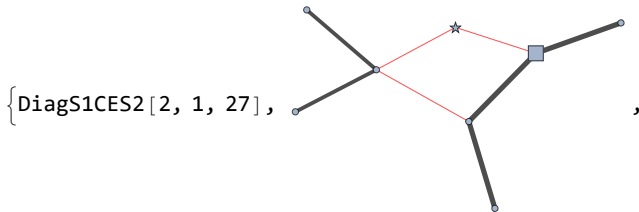

$$\begin{aligned}
G^2 \left( \frac{1}{r^3} \left( \frac{1}{2} \vec{S}_1 \cdot \vec{S}_1 (\hat{n} \cdot \vec{v}_1)^3 - \frac{1}{4} \hat{n} \cdot \vec{S}_1 \vec{S}_1 \cdot \vec{v}_1 (\hat{n} \cdot \vec{v}_1)^2 - 2 \hat{n} \cdot \vec{v}_2 \vec{S}_1 \cdot \vec{S}_1 (\hat{n} \cdot \vec{v}_1)^2 - \right. \right. \\
\left. \frac{1}{4} \hat{n} \cdot \vec{S}_1 \vec{S}_1 \cdot \vec{a}_1 (\hat{n} \cdot \vec{v}_1)^2 - \frac{1}{2} \hat{n} \cdot \vec{a}_1 \vec{S}_1 \cdot \vec{S}_1 (\hat{n} \cdot \vec{v}_1)^2 - \frac{1}{4} \hat{n} \cdot \vec{S}_1 \vec{S}_1 \cdot \vec{v}_1 (\hat{n} \cdot \vec{v}_1)^2 + \right.
\end{aligned}$$



{DiagS1CES2[2, 2, 1],

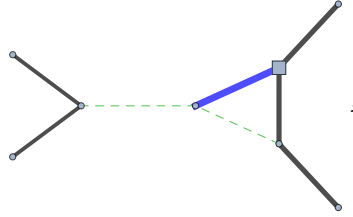

,

$$G^2 \left( \frac{1}{r^2} \left( -16 \vec{v}_1 \cdot \vec{v}_2 \left( \hat{n} \cdot \vec{S}_1 \right)^2 + 8 \vec{S}_1 \cdot \vec{v}_1 \vec{S}_1 \cdot \vec{v}_2 + 4 \vec{S}_1 \cdot \vec{v}_2 \vec{S}_1 \cdot \vec{v}_1 + 4 \vec{S}_1 \cdot \vec{v}_1 \vec{S}_1 \cdot \vec{v}_2 - 16 \hat{n} \cdot \vec{S}_1 \hat{n} \cdot \vec{S}_1 \vec{v}_1 \cdot \vec{v}_2 + \right. \right. \\ \left. \left. 8 \vec{S}_1 \cdot \vec{S}_1 \vec{v}_1 \cdot \vec{v}_2 + 8 \vec{S}_1 \cdot \vec{S}_1 \vec{v}_1 \cdot \vec{v}_2 \right) + \frac{1}{r^3} \left( 8 \hat{n} \cdot \vec{a}_1 \vec{v}_1 \cdot \vec{v}_2 \left( \hat{n} \cdot \vec{S}_1 \right)^2 - 8 \vec{a}_1 \cdot \vec{v}_2 \vec{S}_1 \cdot \vec{v}_1 \hat{n} \cdot \vec{S}_1 - \right. \right. \\ \left. \left. 2 \vec{S}_1 \cdot \vec{v}_2 \vec{v}_1 \cdot \vec{v}_1 \hat{n} \cdot \vec{S}_1 + 32 \hat{n} \cdot \vec{S}_1 \hat{n} \cdot \vec{v}_1 \vec{v}_1 \cdot \vec{v}_2 \hat{n} \cdot \vec{S}_1 - 8 \vec{S}_1 \cdot \vec{v}_1 \vec{v}_1 \cdot \vec{v}_2 \hat{n} \cdot \vec{S}_1 + 4 \vec{S}_1 \cdot \vec{a}_1 \vec{v}_1 \cdot \vec{v}_2 \hat{n} \cdot \vec{S}_1 + \right. \right. \\ \left. \left. 4 \hat{n} \cdot \vec{v}_1 \vec{a}_1 \cdot \vec{v}_2 \vec{S}_1 \cdot \vec{S}_1 + 4 \hat{n} \cdot \vec{v}_2 \vec{S}_1 \cdot \vec{v}_1 \vec{S}_1 \cdot \vec{v}_1 - 2 \hat{n} \cdot \vec{v}_1 \vec{S}_1 \cdot \vec{v}_2 \vec{S}_1 \cdot \vec{v}_1 + 4 \hat{n} \cdot \vec{v}_2 \vec{S}_1 \cdot \vec{a}_1 \vec{S}_1 \cdot \vec{v}_1 - \right. \right. \\ \left. \left. 2 \hat{n} \cdot \vec{v}_1 \vec{S}_1 \cdot \vec{v}_1 \vec{S}_1 \cdot \vec{v}_2 - 4 \hat{n} \cdot \vec{v}_1 \vec{S}_1 \cdot \vec{a}_1 \vec{S}_1 \cdot \vec{v}_2 + 4 \hat{n} \cdot \vec{a}_1 \vec{S}_1 \cdot \vec{v}_1 \vec{S}_1 \cdot \vec{v}_2 + 4 \hat{n} \cdot \vec{v}_2 \vec{S}_1 \cdot \vec{S}_1 \vec{v}_1 \cdot \vec{a}_1 + \right. \right. \\ \left. \left. 8 \hat{n} \cdot \vec{v}_2 \vec{S}_1 \cdot \vec{S}_1 \vec{v}_1 \cdot \vec{v}_1 - 2 \hat{n} \cdot \vec{S}_1 \vec{S}_1 \cdot \vec{v}_2 \vec{v}_1 \cdot \vec{v}_1 + 4 \hat{n} \cdot \vec{v}_1 \vec{S}_1 \cdot \vec{S}_1 \vec{v}_1 \cdot \vec{v}_2 - 8 \hat{n} \cdot \vec{S}_1 \vec{S}_1 \cdot \vec{v}_1 \vec{v}_1 \cdot \vec{v}_2 \right) + \right. \\ \left. \frac{-24 \left( \hat{n} \cdot \vec{v}_1 \right)^2 \vec{v}_1 \cdot \vec{v}_2 \left( \hat{n} \cdot \vec{S}_1 \right)^2 + 4 \vec{v}_1 \cdot \vec{v}_1 \vec{v}_1 \cdot \vec{v}_2 \left( \hat{n} \cdot \vec{S}_1 \right)^2 + 24 \hat{n} \cdot \vec{v}_1 \vec{S}_1 \cdot \vec{v}_1 \vec{v}_1 \cdot \vec{v}_2 \hat{n} \cdot \vec{S}_1 - 4 \left( \vec{S}_1 \cdot \vec{v}_1 \right)^2 \vec{v}_1 \cdot \vec{v}_2}{r^4} \right)$$

$m_2 C_{ES^2_1}$

{DiagS1CES2[2, 2, 2],

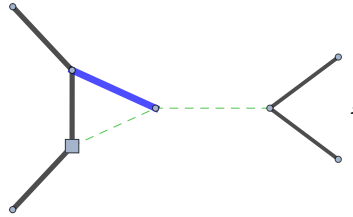

,

$$G^2 m_2 C_{ES^2_1} \left( \frac{1}{r^4} \left( -120 \vec{v}_1 \cdot \vec{v}_2 \left( \hat{n} \cdot \vec{S}_1 \right)^2 \left( \hat{n} \cdot \vec{v}_1 \right)^2 + 20 \vec{v}_1 \cdot \vec{v}_1 \vec{v}_1 \cdot \vec{v}_2 \left( \hat{n} \cdot \vec{S}_1 \right)^2 + \right. \right. \\ \left. \left. 72 \vec{v}_1 \cdot \vec{v}_2 \hat{n} \cdot \vec{S}_1 \hat{n} \cdot \vec{v}_1 \vec{S}_1 \cdot \vec{v}_1 + 16 \vec{S}_1 \cdot \vec{S}_1 \vec{v}_1 \cdot \vec{v}_2 \left( \hat{n} \cdot \vec{v}_1 \right)^2 - 8 \vec{v}_1 \cdot \vec{v}_2 \left( \vec{S}_1 \cdot \vec{v}_1 \right)^2 - 4 \vec{S}_1 \cdot \vec{S}_1 \vec{v}_1 \cdot \vec{v}_1 \vec{v}_1 \cdot \vec{v}_2 \right) + \right. \\ \left. \frac{1}{r^3} \left( 24 \hat{n} \cdot \vec{S}_1 \left( \hat{n} \cdot \vec{v}_1 \right)^2 \vec{S}_1 \cdot \vec{v}_2 - 48 \vec{S}_1 \cdot \vec{S}_1 \hat{n} \cdot \vec{v}_2 \left( \hat{n} \cdot \vec{v}_1 \right)^2 + 24 \hat{n} \cdot \vec{S}_1 \left( \hat{n} \cdot \vec{v}_1 \right)^2 \vec{S}_1 \cdot \vec{v}_2 - \right. \right. \\ \left. \left. 12 \hat{n} \cdot \vec{v}_1 \vec{S}_1 \cdot \vec{v}_2 \vec{S}_1 \cdot \vec{v}_1 - 12 \hat{n} \cdot \vec{v}_1 \vec{S}_1 \cdot \vec{v}_1 \vec{S}_1 \cdot \vec{v}_2 + 28 \vec{S}_1 \cdot \vec{S}_1 \vec{v}_1 \cdot \vec{v}_2 \hat{n} \cdot \vec{v}_1 + \right. \right. \\ \left. \left. 4 \hat{n} \cdot \vec{v}_2 \vec{S}_1 \cdot \vec{v}_1 \vec{S}_1 \cdot \vec{v}_1 + 4 \vec{S}_1 \cdot \vec{S}_1 \vec{v}_1 \cdot \vec{v}_1 \hat{n} \cdot \vec{v}_2 - 6 \vec{v}_1 \cdot \vec{v}_2 \hat{n} \cdot \vec{S}_1 \vec{S}_1 \cdot \vec{v}_1 - 6 \vec{v}_1 \cdot \vec{v}_2 \hat{n} \cdot \vec{S}_1 \vec{S}_1 \cdot \vec{v}_1 \right) \right) \Bigg\}$$

{DiagS1CES2[2, 2, 3],

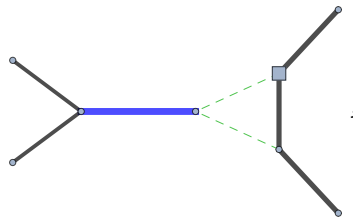

,  $G^2 m_2 C_{ES^2_1}$

$$\left( \frac{1}{r^4} \left( -12 \left( \vec{v}_1 \cdot \vec{v}_2 \right)^2 \left( \hat{n} \cdot \vec{S}_1 \right)^2 + 15 \vec{v}_1 \cdot \vec{v}_1 \left( \hat{n} \cdot \vec{S}_1 \right)^2 \left( \hat{n} \cdot \vec{v}_2 \right)^2 + 7 \vec{v}_1 \cdot \vec{v}_1 \vec{v}_2 \cdot \vec{v}_2 \left( \hat{n} \cdot \vec{S}_1 \right)^2 - 12 \vec{v}_1 \cdot \vec{v}_1 \hat{n} \cdot \vec{S}_1 \hat{n} \cdot \vec{v}_2 \vec{S}_1 \cdot \vec{v}_2 - \right. \right. \\ \left. \left. \vec{S}_1 \cdot \vec{S}_1 \vec{v}_1 \cdot \vec{v}_1 \left( \hat{n} \cdot \vec{v}_2 \right)^2 + 4 \vec{S}_1 \cdot \vec{S}_1 \left( \vec{v}_1 \cdot \vec{v}_2 \right)^2 + 2 \vec{v}_1 \cdot \vec{v}_1 \left( \vec{S}_1 \cdot \vec{v}_2 \right)^2 - 3 \vec{S}_1 \cdot \vec{S}_1 \vec{v}_1 \cdot \vec{v}_1 \vec{v}_2 \cdot \vec{v}_2 \right) + \frac{1}{r^3} \right)$$

$$\left( -4 \hat{n} \cdot \vec{S}_1 \left( \hat{n} \cdot \vec{v}_2 \right)^2 \vec{S}_1 \cdot \vec{v}_1 + 8 \vec{S}_1 \cdot \vec{S}_1 \hat{n} \cdot \vec{v}_1 \left( \hat{n} \cdot \vec{v}_2 \right)^2 - 4 \hat{n} \cdot \vec{S}_1 \left( \hat{n} \cdot \vec{v}_2 \right)^2 \vec{S}_1 \cdot \vec{v}_1 + 4 \hat{n} \cdot \vec{v}_2 \vec{S}_1 \cdot \vec{v}_2 \vec{S}_1 \cdot \vec{v}_1 + \right. \\ \left. 4 \hat{n} \cdot \vec{v}_2 \vec{S}_1 \cdot \vec{v}_1 \vec{S}_1 \cdot \vec{v}_2 - 12 \vec{S}_1 \cdot \vec{S}_1 \vec{v}_1 \cdot \vec{v}_2 \hat{n} \cdot \vec{v}_2 - 4 \hat{n} \cdot \vec{v}_1 \vec{S}_1 \cdot \vec{v}_2 \vec{S}_1 \cdot \vec{v}_2 + 6 \vec{v}_1 \cdot \vec{v}_2 \hat{n} \cdot \vec{S}_1 \vec{S}_1 \cdot \vec{v}_2 + \right. \\ \left. 6 \vec{v}_1 \cdot \vec{v}_2 \hat{n} \cdot \vec{S}_1 \vec{S}_1 \cdot \vec{v}_2 - 4 \vec{v}_2 \cdot \vec{v}_2 \hat{n} \cdot \vec{S}_1 \vec{S}_1 \cdot \vec{v}_1 + 4 \vec{S}_1 \cdot \vec{S}_1 \vec{v}_2 \cdot \vec{v}_2 \hat{n} \cdot \vec{v}_1 - 4 \vec{v}_2 \cdot \vec{v}_2 \hat{n} \cdot \vec{S}_1 \vec{S}_1 \cdot \vec{v}_1 \right) \Bigg\}$$

$$\left\{ \text{DiagS1CES2}[2, 2, 4], \frac{1}{m_1} \right\}$$

$$G^2 m_2^2 C_{\text{ES}^2 1} \left( \frac{1}{r^3} \left( -4 \vec{v}_2 \cdot \vec{v}_2 \hat{n} \cdot \vec{a}_1 \left( \hat{n} \cdot \vec{S}_1 \right)^2 + 8 \vec{a}_1 \cdot \vec{v}_2 \hat{n} \cdot \vec{S}_1 \vec{S}_1 \cdot \vec{v}_2 - 4 \vec{v}_2 \cdot \vec{v}_2 \vec{S}_1 \cdot \vec{a}_1 \hat{n} \cdot \vec{S}_1 - 4 \hat{n} \cdot \vec{a}_1 \left( \vec{S}_1 \cdot \vec{v}_2 \right)^2 - \right. \right. \\ \left. \left. 8 \vec{S}_1 \cdot \vec{S}_1 \vec{a}_1 \cdot \vec{v}_2 \hat{n} \cdot \vec{v}_2 + 4 \vec{S}_1 \cdot \vec{S}_1 \vec{v}_2 \cdot \vec{v}_2 \hat{n} \cdot \vec{a}_1 + 8 \vec{v}_1 \cdot \vec{v}_2 \hat{n} \cdot \vec{S}_1 \vec{S}_1 \cdot \vec{v}_2 - 16 \vec{v}_2 \cdot \vec{v}_2 \hat{n} \cdot \vec{S}_1 \hat{n} \cdot \vec{S}_1 \hat{n} \cdot \vec{v}_1 - 2 \vec{v}_2 \cdot \vec{v}_2 \right. \right. \\ \left. \left. \hat{n} \cdot \vec{S}_1 \vec{S}_1 \cdot \vec{v}_1 - 16 \vec{S}_1 \cdot \vec{S}_1 \vec{v}_1 \cdot \vec{v}_2 \hat{n} \cdot \vec{v}_2 + 8 \vec{v}_1 \cdot \vec{v}_2 \hat{n} \cdot \vec{S}_1 \vec{S}_1 \cdot \vec{v}_2 + 12 \vec{S}_1 \cdot \vec{S}_1 \vec{v}_2 \cdot \vec{v}_2 \hat{n} \cdot \vec{v}_1 - 2 \vec{v}_2 \cdot \vec{v}_2 \hat{n} \cdot \vec{S}_1 \vec{S}_1 \cdot \vec{v}_1 \right) + \right. \\ \left. \frac{1}{r^4} \left( -16 \left( \vec{v}_1 \cdot \vec{v}_2 \right)^2 \left( \hat{n} \cdot \vec{S}_1 \right)^2 + 24 \vec{v}_2 \cdot \vec{v}_2 \left( \hat{n} \cdot \vec{S}_1 \right)^2 \left( \hat{n} \cdot \vec{v}_1 \right)^2 + 8 \vec{v}_1 \cdot \vec{v}_1 \vec{v}_2 \cdot \vec{v}_2 \left( \hat{n} \cdot \vec{S}_1 \right)^2 - \right. \right. \\ \left. \left. 16 \vec{v}_2 \cdot \vec{v}_2 \hat{n} \cdot \vec{S}_1 \hat{n} \cdot \vec{v}_1 \vec{S}_1 \cdot \vec{v}_1 + 8 \vec{S}_1 \cdot \vec{S}_1 \left( \vec{v}_1 \cdot \vec{v}_2 \right)^2 + 2 \vec{v}_2 \cdot \vec{v}_2 \left( \vec{S}_1 \cdot \vec{v}_1 \right)^2 - 6 \vec{S}_1 \cdot \vec{S}_1 \vec{v}_1 \cdot \vec{v}_1 \vec{v}_2 \cdot \vec{v}_2 \right) + \right. \\ \left. \left. 2 \vec{v}_2 \cdot \vec{v}_2 \left( \hat{n} \cdot \vec{S}_1 \right)^2 + 2 \vec{v}_2 \cdot \vec{v}_2 \hat{n} \cdot \vec{S}_1 \hat{n} \cdot \vec{S}_1 - 4 \left( \frac{1}{\vec{S}_1 \cdot \vec{v}_2} \right)^2 - 4 \frac{2}{\vec{S}_1 \cdot \vec{v}_2} \vec{S}_1 \cdot \vec{v}_2 - 2 \frac{1}{\vec{S}_1 \cdot \vec{S}_1} \vec{v}_2 \cdot \vec{v}_2 - 2 \vec{S}_1 \cdot \vec{S}_1 \vec{v}_2 \cdot \vec{v}_2 \right) \right) \Bigg\}$$

$$\left\{ \text{DiagS1CES2}[2, 2, 5], \frac{1}{m_1} G^2 m_2^2 C_{\text{ES}^2 1} \right\}$$

$$\left( \frac{-192 \vec{v}_1 \cdot \vec{v}_2 \left( \hat{n} \cdot \vec{S}_1 \right)^2 \left( \hat{n} \cdot \vec{v}_2 \right)^2 + 32 \vec{v}_1 \cdot \vec{v}_2 \vec{v}_2 \cdot \vec{v}_2 \left( \hat{n} \cdot \vec{S}_1 \right)^2 + 128 \vec{v}_1 \cdot \vec{v}_2 \hat{n} \cdot \vec{S}_1 \hat{n} \cdot \vec{v}_2 \vec{S}_1 \cdot \vec{v}_2 - 16 \vec{v}_1 \cdot \vec{v}_2 \left( \vec{S}_1 \cdot \vec{v}_2 \right)^2}{r^4} + \right. \\ \left. \frac{1}{r^3} \left( -64 \vec{S}_1 \cdot \vec{S}_1 \left( \hat{n} \cdot \vec{v}_2 \right)^3 + 32 \hat{n} \cdot \vec{S}_1 \left( \hat{n} \cdot \vec{v}_2 \right)^2 \vec{S}_1 \cdot \vec{v}_2 + 32 \hat{n} \cdot \vec{S}_1 \left( \hat{n} \cdot \vec{v}_2 \right)^2 \vec{S}_1 \cdot \vec{v}_2 - \right. \right. \\ \left. \left. 32 \hat{n} \cdot \vec{v}_2 \vec{S}_1 \cdot \vec{v}_2 \vec{S}_1 \cdot \vec{v}_2 + 48 \vec{S}_1 \cdot \vec{S}_1 \vec{v}_2 \cdot \vec{v}_2 \hat{n} \cdot \vec{v}_2 - 8 \vec{v}_2 \cdot \vec{v}_2 \hat{n} \cdot \vec{S}_1 \vec{S}_1 \cdot \vec{v}_2 - 8 \vec{v}_2 \cdot \vec{v}_2 \hat{n} \cdot \vec{S}_1 \vec{S}_1 \cdot \vec{v}_2 \right) \right) \Bigg\}$$

$$\left\{ \text{DiagS1CES2}[2, 2, 6], \right\}$$

$$\begin{aligned} & \mathcal{G}^2 \left( \frac{1}{r^2} \left( -12 \hat{n} \cdot \vec{v}_1 \hat{n} \cdot \vec{v}_2 \vec{S}_1 \cdot \vec{S}_1 + 4 \vec{v}_1 \cdot \vec{v}_2 \vec{S}_1 \cdot \vec{S}_1 - 6 \hat{n} \cdot \vec{S}_1 \hat{n} \cdot \vec{v}_2 \vec{S}_1 \cdot \vec{a}_1 - 6 \hat{n} \cdot \vec{S}_1 \hat{n} \cdot \vec{v}_1 \vec{S}_1 \cdot \vec{a}_2 - 4 \hat{n} \cdot \vec{S}_1 \hat{n} \cdot \vec{v}_2 \vec{S}_1 \cdot \vec{v}_1 + \right. \right. \\ & 16 \hat{n} \cdot \vec{S}_1 \hat{n} \cdot \vec{v}_1 \vec{S}_1 \cdot \vec{v}_2 - 4 \vec{S}_1 \cdot \vec{v}_1 \vec{S}_1 \cdot \vec{v}_2 - 2 \hat{n} \cdot \vec{S}_1 \hat{n} \cdot \vec{v}_2 \vec{S}_1 \cdot \vec{v}_1 + 8 \hat{n} \cdot \vec{S}_1 \hat{n} \cdot \vec{v}_1 \vec{S}_1 \cdot \vec{v}_2 + 16 \hat{n} \cdot \vec{S}_1 \hat{n} \cdot \vec{S}_1 \vec{a}_1 \cdot \vec{v}_2 + \\ & 12 \hat{n} \cdot \vec{a}_2 \hat{n} \cdot \vec{v}_1 \vec{S}_1 \cdot \vec{S}_1 + 12 \hat{n} \cdot \vec{a}_1 \hat{n} \cdot \vec{v}_2 \vec{S}_1 \cdot \vec{S}_1 - 4 \vec{a}_1 \cdot \vec{v}_2 \vec{S}_1 \cdot \vec{S}_1 - 12 \hat{n} \cdot \vec{v}_1 \hat{n} \cdot \vec{v}_2 \vec{S}_1 \cdot \vec{S}_1 - 6 \hat{n} \cdot \vec{S}_1 \hat{n} \cdot \vec{v}_2 \vec{S}_1 \cdot \vec{a}_1 + \\ & 2 \vec{S}_1 \cdot \vec{v}_2 \vec{S}_1 \cdot \vec{a}_1 - 6 \hat{n} \cdot \vec{S}_1 \hat{n} \cdot \vec{v}_1 \vec{S}_1 \cdot \vec{a}_2 + 2 \vec{S}_1 \cdot \vec{v}_1 \vec{S}_1 \cdot \vec{a}_2 - 2 \hat{n} \cdot \vec{S}_1 \hat{n} \cdot \vec{v}_2 \vec{S}_1 \cdot \vec{v}_1 + 2 \vec{S}_1 \cdot \vec{a}_2 \vec{S}_1 \cdot \vec{v}_1 - 2 \vec{S}_1 \cdot \vec{v}_2 \vec{S}_1 \cdot \vec{v}_1 + \\ & 8 \hat{n} \cdot \vec{S}_1 \hat{n} \cdot \vec{v}_1 \vec{S}_1 \cdot \vec{v}_2 + 2 \vec{S}_1 \cdot \vec{a}_1 \vec{S}_1 \cdot \vec{v}_2 - 2 \vec{S}_1 \cdot \vec{v}_1 \vec{S}_1 \cdot \vec{v}_2 - 4 \hat{n} \cdot \vec{S}_1 \hat{n} \cdot \vec{S}_1 \vec{v}_1 \cdot \vec{a}_2 - 8 \vec{S}_1 \cdot \vec{S}_1 \vec{v}_1 \cdot \vec{a}_2 + 4 \vec{S}_1 \cdot \vec{S}_1 \vec{v}_1 \cdot \vec{v}_2 \Big) + \\ & \frac{1}{r^4} \left( -24 (\vec{v}_1 \cdot \vec{v}_2)^2 (\hat{n} \cdot \vec{S}_1)^2 - 30 \hat{n} \cdot \vec{v}_1 \hat{n} \cdot \vec{v}_2 \vec{v}_1 \cdot \vec{v}_1 (\hat{n} \cdot \vec{S}_1)^2 + 144 (\hat{n} \cdot \vec{v}_1)^2 \vec{v}_1 \cdot \vec{v}_2 (\hat{n} \cdot \vec{S}_1)^2 + \right. \\ & 144 \hat{n} \cdot \vec{v}_1 \hat{n} \cdot \vec{v}_2 \vec{v}_1 \cdot \vec{v}_2 (\hat{n} \cdot \vec{S}_1)^2 - 14 \vec{v}_1 \cdot \vec{v}_1 \vec{v}_1 \cdot \vec{v}_2 (\hat{n} \cdot \vec{S}_1)^2 + 12 \hat{n} \cdot \vec{v}_2 \vec{S}_1 \cdot \vec{v}_1 \vec{v}_1 \cdot \vec{v}_1 \hat{n} \cdot \vec{S}_1 + 12 \hat{n} \cdot \vec{v}_1 \vec{S}_1 \cdot \vec{v}_2 \\ & \vec{v}_1 \cdot \vec{v}_1 \hat{n} \cdot \vec{S}_1 - 96 \hat{n} \cdot \vec{v}_1 \vec{S}_1 \cdot \vec{v}_1 \vec{v}_1 \cdot \vec{v}_2 \hat{n} \cdot \vec{S}_1 - 48 \hat{n} \cdot \vec{v}_2 \vec{S}_1 \cdot \vec{v}_1 \vec{v}_1 \cdot \vec{v}_2 \hat{n} \cdot \vec{S}_1 - 48 \hat{n} \cdot \vec{v}_1 \vec{S}_1 \cdot \vec{v}_2 \vec{v}_1 \cdot \vec{v}_2 \hat{n} \cdot \vec{S}_1 + \\ & 4 \vec{S}_1 \cdot \vec{S}_1 (\vec{v}_1 \cdot \vec{v}_2)^2 + 2 \hat{n} \cdot \vec{v}_1 \hat{n} \cdot \vec{v}_2 \vec{S}_1 \cdot \vec{S}_1 \vec{v}_1 \cdot \vec{v}_1 - 4 \vec{S}_1 \cdot \vec{v}_1 \vec{S}_1 \cdot \vec{v}_2 \vec{v}_1 \cdot \vec{v}_1 + 12 (\vec{S}_1 \cdot \vec{v}_1)^2 \vec{v}_1 \cdot \vec{v}_2 - \\ & 16 (\hat{n} \cdot \vec{v}_1)^2 \vec{S}_1 \cdot \vec{S}_1 \vec{v}_1 \cdot \vec{v}_2 - 16 \hat{n} \cdot \vec{v}_1 \hat{n} \cdot \vec{v}_2 \vec{S}_1 \cdot \vec{S}_1 \vec{v}_1 \cdot \vec{v}_2 + 12 \vec{S}_1 \cdot \vec{v}_1 \vec{S}_1 \cdot \vec{v}_2 \vec{v}_1 \cdot \vec{v}_2 + 2 \vec{S}_1 \cdot \vec{S}_1 \vec{v}_1 \cdot \vec{v}_1 \vec{v}_1 \cdot \vec{v}_2 \Big) + \frac{1}{r^3} \\ & \left( -48 \hat{n} \cdot \vec{v}_1 \vec{a}_1 \cdot \vec{v}_2 (\hat{n} \cdot \vec{S}_1)^2 + 24 \hat{n} \cdot \vec{v}_2 \vec{v}_1 \cdot \vec{a}_1 (\hat{n} \cdot \vec{S}_1)^2 + 24 \hat{n} \cdot \vec{v}_1 \vec{v}_1 \cdot \vec{a}_2 (\hat{n} \cdot \vec{S}_1)^2 + 8 \hat{n} \cdot \vec{v}_1 \hat{n} \cdot \vec{v}_2 \vec{S}_1 \cdot \vec{v}_1 \hat{n} \cdot \vec{S}_1 - \right. \\ & 24 (\hat{n} \cdot \vec{v}_1)^2 \vec{S}_1 \cdot \vec{v}_2 \hat{n} \cdot \vec{S}_1 - 24 \hat{n} \cdot \vec{v}_1 \hat{n} \cdot \vec{v}_2 \vec{S}_1 \cdot \vec{v}_2 \hat{n} \cdot \vec{S}_1 + 24 \vec{a}_1 \cdot \vec{v}_2 \vec{S}_1 \cdot \vec{v}_1 \hat{n} \cdot \vec{S}_1 - 12 \vec{S}_1 \cdot \vec{v}_2 \vec{v}_1 \cdot \vec{a}_1 \hat{n} \cdot \vec{S}_1 - \\ & 12 \vec{S}_1 \cdot \vec{v}_1 \vec{v}_1 \cdot \vec{a}_2 \hat{n} \cdot \vec{S}_1 + 8 \hat{n} \cdot \vec{S}_1 \hat{n} \cdot \vec{v}_2 \vec{v}_1 \cdot \vec{v}_1 \hat{n} \cdot \vec{S}_1 + 2 \vec{S}_1 \cdot \vec{v}_2 \vec{v}_1 \cdot \vec{v}_1 \hat{n} \cdot \vec{S}_1 - 64 \hat{n} \cdot \vec{S}_1 \hat{n} \cdot \vec{v}_1 \vec{v}_1 \cdot \vec{v}_2 \hat{n} \cdot \vec{S}_1 - \\ & 16 \hat{n} \cdot \vec{S}_1 \hat{n} \cdot \vec{v}_2 \vec{v}_1 \cdot \vec{v}_2 \hat{n} \cdot \vec{S}_1 + 14 \vec{S}_1 \cdot \vec{v}_1 \vec{v}_1 \cdot \vec{v}_2 \hat{n} \cdot \vec{S}_1 + 10 \vec{S}_1 \cdot \vec{v}_2 \vec{v}_1 \cdot \vec{v}_2 \hat{n} \cdot \vec{S}_1 + 48 \hat{n} \cdot \vec{v}_1 (\hat{n} \cdot \vec{v}_2)^2 \vec{S}_1 \cdot \vec{S}_1 + \\ & 32 (\hat{n} \cdot \vec{v}_1)^2 \hat{n} \cdot \vec{v}_2 \vec{S}_1 \cdot \vec{S}_1 + 8 \hat{n} \cdot \vec{v}_1 \vec{a}_1 \cdot \vec{v}_2 \vec{S}_1 \cdot \vec{S}_1 + 8 \hat{n} \cdot \vec{S}_1 \hat{n} \cdot \vec{v}_1 \hat{n} \cdot \vec{v}_2 \vec{S}_1 \cdot \vec{v}_1 - 4 \hat{n} \cdot \vec{v}_2 \vec{S}_1 \cdot \vec{v}_1 \vec{S}_1 \cdot \vec{v}_1 + \\ & 8 \hat{n} \cdot \vec{v}_1 \vec{S}_1 \cdot \vec{v}_2 \vec{S}_1 \cdot \vec{v}_1 + 4 \hat{n} \cdot \vec{v}_2 \vec{S}_1 \cdot \vec{v}_2 \vec{S}_1 \cdot \vec{v}_1 - 24 \hat{n} \cdot \vec{S}_1 (\hat{n} \cdot \vec{v}_1)^2 \vec{S}_1 \cdot \vec{v}_2 - 24 \hat{n} \cdot \vec{S}_1 \hat{n} \cdot \vec{v}_1 \hat{n} \cdot \vec{v}_2 \vec{S}_1 \cdot \vec{v}_2 + \\ & 8 \hat{n} \cdot \vec{v}_1 \vec{S}_1 \cdot \vec{v}_1 \vec{S}_1 \cdot \vec{v}_2 + 4 \hat{n} \cdot \vec{v}_2 \vec{S}_1 \cdot \vec{v}_1 \vec{S}_1 \cdot \vec{v}_2 + 12 \hat{n} \cdot \vec{v}_1 \vec{S}_1 \cdot \vec{v}_2 \vec{S}_1 \cdot \vec{v}_2 - 4 \hat{n} \cdot \vec{v}_2 \vec{S}_1 \cdot \vec{S}_1 \vec{v}_1 \cdot \vec{a}_1 - \\ & 4 \hat{n} \cdot \vec{v}_1 \vec{S}_1 \cdot \vec{S}_1 \vec{v}_1 \cdot \vec{a}_2 - 8 \hat{n} \cdot \vec{v}_2 \vec{S}_1 \cdot \vec{S}_1 \vec{v}_1 \cdot \vec{v}_1 + 2 \hat{n} \cdot \vec{S}_1 \vec{S}_1 \cdot \vec{v}_2 \vec{v}_1 \cdot \vec{v}_1 - 4 \hat{n} \cdot \vec{v}_1 \vec{S}_1 \cdot \vec{S}_1 \vec{v}_1 \cdot \vec{v}_2 - \\ & 28 \hat{n} \cdot \vec{v}_2 \vec{S}_1 \cdot \vec{S}_1 \vec{v}_1 \cdot \vec{v}_2 + 14 \hat{n} \cdot \vec{S}_1 \vec{S}_1 \cdot \vec{v}_1 \vec{v}_1 \cdot \vec{v}_2 + 10 \hat{n} \cdot \vec{S}_1 \vec{S}_1 \cdot \vec{v}_2 \vec{v}_1 \cdot \vec{v}_2 - 12 \hat{n} \cdot \vec{v}_1 \vec{S}_1 \cdot \vec{S}_1 \vec{v}_2 \cdot \vec{v}_2 \Big) \Big) m_2 C_{\text{ES}^2_1} \} \end{aligned}$$

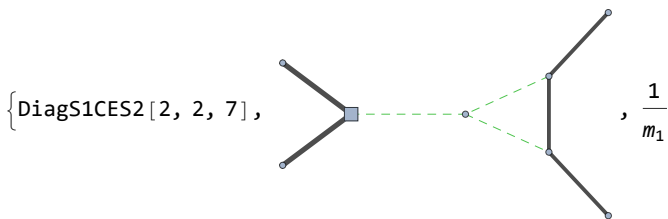

$$\begin{aligned} G^2 & \left( \frac{1}{r^2} \left( -16 \vec{S_1}^1 \cdot \vec{S_1}^1 (\hat{n} \cdot \vec{v_2})^2 - 16 \vec{S_1}^1 \cdot \vec{S_1}^2 (\hat{n} \cdot \vec{v_2})^2 - 16 \hat{n} \cdot \vec{S_1}^1 \vec{S_1}^1 \cdot \vec{a_2} \hat{n} \cdot \vec{v_2} + 16 \hat{n} \cdot \vec{S_1}^1 \vec{S_1}^1 \cdot \vec{v_2} \hat{n} \cdot \vec{v_2} + 8 \hat{n} \cdot \vec{S_1}^1 \vec{S_1}^2 \cdot \vec{v_2} \hat{n} \cdot \vec{v_2} + \right. \right. \\ & 32 \hat{n} \cdot \vec{a_2} \vec{S_1}^1 \cdot \vec{S_1}^1 \hat{n} \cdot \vec{v_2} - 16 \hat{n} \cdot \vec{S_1}^1 \vec{S_1}^1 \cdot \vec{a_2} \hat{n} \cdot \vec{v_2} + 8 \hat{n} \cdot \vec{S_1}^2 \vec{S_1}^1 \cdot \vec{v_2} \hat{n} \cdot \vec{v_2} - 8 \left( \frac{1}{\vec{S_1}^1 \cdot \vec{v_2}} \right)^2 + 8 \vec{S_1}^1 \cdot \vec{v_2} \vec{S_1}^1 \cdot \vec{a_2} + \\ & 8 \vec{S_1}^1 \cdot \vec{a_2} \vec{S_1}^1 \cdot \vec{v_2} - 8 \vec{S_1}^2 \cdot \vec{v_2} \vec{S_1}^1 \cdot \vec{v_2} + 16 \hat{n} \cdot \vec{S_1}^1 \hat{n} \cdot \vec{S_1}^1 \vec{v_2} \cdot \vec{a_2} - 16 \vec{S_1}^1 \cdot \vec{S_1}^1 \vec{v_2} \cdot \vec{a_2} + 8 \vec{S_1}^1 \cdot \vec{S_1}^1 \vec{v_2} \cdot \vec{v_2} + 8 \vec{S_1}^1 \cdot \vec{S_1}^2 \vec{v_2} \cdot \vec{v_2} \Big) + \\ & \frac{1}{r^3} \left( 64 \vec{S_1}^1 \cdot \vec{S_1}^1 (\hat{n} \cdot \vec{v_2})^3 - 32 \hat{n} \cdot \vec{S_1}^1 \vec{S_1}^1 \cdot \vec{v_2} (\hat{n} \cdot \vec{v_2})^2 + 64 \hat{n} \cdot \vec{v_1} \vec{S_1}^1 \cdot \vec{S_1}^1 (\hat{n} \cdot \vec{v_2})^2 - 32 \hat{n} \cdot \vec{S_1}^1 \vec{S_1}^1 \cdot \vec{v_2} (\hat{n} \cdot \vec{v_2})^2 - \right. \\ & 32 \hat{n} \cdot \vec{S_1}^1 \hat{n} \cdot \vec{v_1} \vec{S_1}^1 \cdot \vec{v_2} \hat{n} \cdot \vec{v_2} - 32 (\hat{n} \cdot \vec{S_1}^1)^2 \vec{a_1} \cdot \vec{v_2} \hat{n} \cdot \vec{v_2} + 8 \vec{S_1}^1 \cdot \vec{v_2} \vec{S_1}^1 \cdot \vec{v_1} \hat{n} \cdot \vec{v_2} - 32 \hat{n} \cdot \vec{S_1}^1 \hat{n} \cdot \vec{v_1} \vec{S_1}^1 \cdot \vec{v_2} \hat{n} \cdot \vec{v_2} + \\ & 8 \vec{S_1}^1 \cdot \vec{v_1} \vec{S_1}^1 \cdot \vec{v_2} \hat{n} \cdot \vec{v_2} + 32 \vec{S_1}^1 \cdot \vec{v_2} \vec{S_1}^1 \cdot \vec{v_2} \hat{n} \cdot \vec{v_2} + 64 (\hat{n} \cdot \vec{S_1}^1)^2 \vec{v_1} \cdot \vec{a_2} \hat{n} \cdot \vec{v_2} - 64 \hat{n} \cdot \vec{S_1}^1 \hat{n} \cdot \vec{S_1}^1 \vec{v_1} \cdot \vec{v_2} \hat{n} \cdot \vec{v_2} - \\ & \left. 32 \vec{S_1}^1 \cdot \vec{S_1}^1 \vec{v_1} \cdot \vec{v_2} \hat{n} \cdot \vec{v_2} + 16 \hat{n} \cdot \vec{S_1}^1 \hat{n} \cdot \vec{S_1}^1 \vec{v_2} \cdot \vec{v_2} \hat{n} \cdot \vec{v_2} - 44 \vec{S_1}^1 \cdot \vec{S_1}^1 \vec{v_2} \cdot \vec{v_2} \hat{n} \cdot \vec{v_2} + 16 \hat{n} \cdot \vec{v_1} \vec{S_1}^1 \cdot \vec{v_2} \vec{S_1}^1 \cdot \vec{v_2} + \right. \end{aligned}$$

$$\begin{aligned}
& 16 \hat{n} \cdot \vec{S}_1 \vec{a}_1 \cdot \vec{v}_2 \vec{S}_1 \cdot \vec{v}_2 - 32 \hat{n} \cdot \vec{S}_1 \vec{S}_1 \cdot \vec{v}_2 \vec{v}_1 \cdot \vec{a}_2 + 24 \hat{n} \cdot \vec{S}_1 \vec{S}_1 \cdot \vec{v}_2 \vec{v}_1 \cdot \vec{v}_2 + 24 \hat{n} \cdot \vec{S}_1 \vec{S}_1 \cdot \vec{v}_2 \vec{v}_1 \cdot \vec{v}_2 - 32 \left( \hat{n} \cdot \vec{S}_1 \right)^2 \\
& \hat{n} \cdot \vec{v}_1 \vec{v}_2 \cdot \vec{a}_2 + 16 \hat{n} \cdot \vec{S}_1 \vec{S}_1 \cdot \vec{v}_1 \vec{v}_2 \cdot \vec{a}_2 + 2 \hat{n} \cdot \vec{S}_1 \vec{S}_1 \cdot \vec{v}_2 \vec{v}_2 \cdot \vec{v}_2 - 16 \hat{n} \cdot \vec{v}_1 \vec{S}_1 \cdot \vec{S}_1 \vec{v}_2 \cdot \vec{v}_2 + 2 \hat{n} \cdot \vec{S}_1 \vec{S}_1 \cdot \vec{v}_2 \vec{v}_2 \cdot \vec{v}_2 \Big) + \\
& \frac{1}{r^4} \left( -32 \left( \vec{v}_1 \cdot \vec{v}_2 \right)^2 \left( \hat{n} \cdot \vec{S}_1 \right)^2 + 192 \left( \hat{n} \cdot \vec{v}_2 \right)^2 \vec{v}_1 \cdot \vec{v}_2 \left( \hat{n} \cdot \vec{S}_1 \right)^2 + 192 \hat{n} \cdot \vec{v}_1 \hat{n} \cdot \vec{v}_2 \vec{v}_1 \cdot \vec{v}_2 \left( \hat{n} \cdot \vec{S}_1 \right)^2 - \right. \\
& 48 \hat{n} \cdot \vec{v}_1 \hat{n} \cdot \vec{v}_2 \vec{v}_2 \cdot \vec{v}_2 \left( \hat{n} \cdot \vec{S}_1 \right)^2 - 16 \vec{v}_1 \cdot \vec{v}_2 \vec{v}_2 \cdot \vec{v}_2 \left( \hat{n} \cdot \vec{S}_1 \right)^2 - 64 \hat{n} \cdot \vec{v}_2 \vec{S}_1 \cdot \vec{v}_1 \vec{v}_1 \cdot \vec{v}_2 \hat{n} \cdot \vec{S}_1 - 64 \hat{n} \cdot \vec{v}_1 \vec{S}_1 \cdot \vec{v}_2 \\
& \vec{v}_1 \cdot \vec{v}_2 \hat{n} \cdot \vec{S}_1 - 128 \hat{n} \cdot \vec{v}_2 \vec{S}_1 \cdot \vec{v}_2 \vec{v}_1 \cdot \vec{v}_2 \hat{n} \cdot \vec{S}_1 + 16 \hat{n} \cdot \vec{v}_2 \vec{S}_1 \cdot \vec{v}_1 \vec{v}_2 \cdot \vec{v}_2 \hat{n} \cdot \vec{S}_1 + 16 \hat{n} \cdot \vec{v}_1 \vec{S}_1 \cdot \vec{v}_2 \vec{v}_2 \cdot \vec{v}_2 \hat{n} \cdot \vec{S}_1 + \\
& \left. 16 \left( \vec{S}_1 \cdot \vec{v}_2 \right)^2 \vec{v}_1 \cdot \vec{v}_2 + 16 \vec{S}_1 \cdot \vec{v}_1 \vec{S}_1 \cdot \vec{v}_2 \vec{v}_1 \cdot \vec{v}_2 - 4 \vec{S}_1 \cdot \vec{v}_1 \vec{S}_1 \cdot \vec{v}_2 \vec{v}_2 \cdot \vec{v}_2 - 4 \vec{S}_1 \cdot \vec{S}_1 \vec{v}_1 \cdot \vec{v}_2 \vec{v}_2 \cdot \vec{v}_2 \right) \Big) m_{\text{CES}^2}^2 \Big\}
\end{aligned}$$

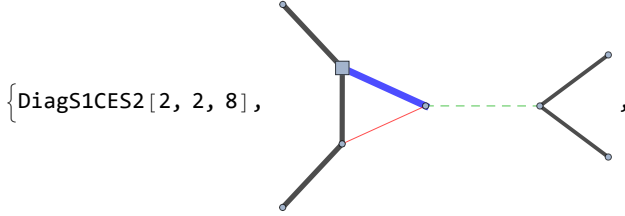

$$\begin{aligned}
& G^2 \left( \frac{8 \hat{n} \cdot \vec{a}_2 \vec{S}_1 \cdot \vec{S}_1 - 8 \hat{n} \cdot \vec{S}_1 \vec{S}_1 \cdot \vec{a}_2 - 4 \hat{n} \cdot \vec{S}_1 \vec{S}_1 \cdot \vec{a}_2 + 8 \hat{n} \cdot \vec{a}_2 \vec{S}_1 \cdot \vec{S}_1 - 4 \hat{n} \cdot \vec{S}_1 \vec{S}_1 \cdot \vec{a}_2}{r} + \right. \\
& \frac{1}{r^4} \left( 4 \left( \vec{v}_1 \cdot \vec{v}_2 \right)^2 \left( \hat{n} \cdot \vec{S}_1 \right)^2 + 24 \left( \hat{n} \cdot \vec{v}_1 \right)^2 \vec{v}_1 \cdot \vec{v}_2 \left( \hat{n} \cdot \vec{S}_1 \right)^2 - 24 \hat{n} \cdot \vec{v}_1 \hat{n} \cdot \vec{v}_2 \vec{v}_1 \cdot \vec{v}_2 \left( \hat{n} \cdot \vec{S}_1 \right)^2 - \right. \\
& 4 \vec{v}_1 \cdot \vec{v}_1 \vec{v}_1 \cdot \vec{v}_2 \left( \hat{n} \cdot \vec{S}_1 \right)^2 - 24 \hat{n} \cdot \vec{v}_1 \vec{S}_1 \cdot \vec{v}_1 \vec{v}_1 \cdot \vec{v}_2 \hat{n} \cdot \vec{S}_1 + 16 \hat{n} \cdot \vec{v}_2 \vec{S}_1 \cdot \vec{v}_1 \vec{v}_1 \cdot \vec{v}_2 \hat{n} \cdot \vec{S}_1 + \\
& 8 \hat{n} \cdot \vec{v}_1 \vec{S}_1 \cdot \vec{v}_2 \vec{v}_1 \cdot \vec{v}_2 \hat{n} \cdot \vec{S}_1 + 4 \left( \vec{S}_1 \cdot \vec{v}_1 \right)^2 \vec{v}_1 \cdot \vec{v}_2 - 4 \vec{S}_1 \cdot \vec{v}_1 \vec{S}_1 \cdot \vec{v}_2 \vec{v}_1 \cdot \vec{v}_2 \Big) + \frac{1}{r^3} \\
& \left( -8 \hat{n} \cdot \vec{v}_1 \vec{a}_1 \cdot \vec{v}_2 \left( \hat{n} \cdot \vec{S}_1 \right)^2 + 8 \hat{n} \cdot \vec{v}_2 \vec{a}_1 \cdot \vec{v}_2 \left( \hat{n} \cdot \vec{S}_1 \right)^2 - 4 \hat{n} \cdot \vec{v}_1 \vec{v}_1 \cdot \vec{a}_2 \left( \hat{n} \cdot \vec{S}_1 \right)^2 - 8 \left( \hat{n} \cdot \vec{v}_1 \right)^2 \vec{S}_1 \cdot \vec{v}_2 \hat{n} \cdot \vec{S}_1 + \right. \\
& 8 \hat{n} \cdot \vec{v}_1 \hat{n} \cdot \vec{v}_2 \vec{S}_1 \cdot \vec{v}_2 \hat{n} \cdot \vec{S}_1 + 6 \vec{a}_1 \cdot \vec{v}_2 \vec{S}_1 \cdot \vec{v}_1 \hat{n} \cdot \vec{S}_1 - 4 \vec{a}_1 \cdot \vec{v}_2 \vec{S}_1 \cdot \vec{v}_2 \hat{n} \cdot \vec{S}_1 - 2 \vec{S}_1 \cdot \vec{v}_2 \vec{v}_1 \cdot \vec{a}_1 \hat{n} \cdot \vec{S}_1 + \\
& 4 \vec{S}_1 \cdot \vec{v}_1 \vec{v}_1 \cdot \vec{a}_2 \hat{n} \cdot \vec{S}_1 + 2 \vec{S}_1 \cdot \vec{v}_2 \vec{v}_1 \cdot \vec{v}_1 \hat{n} \cdot \vec{S}_1 - 16 \hat{n} \cdot \vec{S}_1 \hat{n} \cdot \vec{v}_1 \vec{v}_1 \cdot \vec{v}_2 \hat{n} \cdot \vec{S}_1 + 16 \hat{n} \cdot \vec{S}_1 \hat{n} \cdot \vec{v}_2 \vec{v}_1 \cdot \vec{v}_2 \hat{n} \cdot \vec{S}_1 + \\
& 6 \vec{S}_1 \cdot \vec{v}_1 \vec{v}_1 \cdot \vec{v}_2 \hat{n} \cdot \vec{S}_1 - 6 \vec{S}_1 \cdot \vec{v}_2 \vec{v}_1 \cdot \vec{v}_2 \hat{n} \cdot \vec{S}_1 - 16 \hat{n} \cdot \vec{v}_1 \left( \hat{n} \cdot \vec{v}_2 \right)^2 \vec{S}_1 \cdot \vec{S}_1 + 16 \left( \hat{n} \cdot \vec{v}_1 \right)^2 \hat{n} \cdot \vec{v}_2 \vec{S}_1 \cdot \vec{S}_1 - \\
& 2 \hat{n} \cdot \vec{v}_1 \vec{a}_1 \cdot \vec{v}_2 \vec{S}_1 \cdot \vec{S}_1 + 4 \hat{n} \cdot \vec{v}_2 \vec{a}_1 \cdot \vec{v}_2 \vec{S}_1 \cdot \vec{S}_1 + 6 \hat{n} \cdot \vec{v}_1 \vec{S}_1 \cdot \vec{v}_2 \vec{S}_1 \cdot \vec{v}_1 - 4 \hat{n} \cdot \vec{v}_2 \vec{S}_1 \cdot \vec{v}_2 \vec{S}_1 \cdot \vec{v}_1 - \\
& 8 \hat{n} \cdot \vec{S}_1 \left( \hat{n} \cdot \vec{v}_1 \right)^2 \vec{S}_1 \cdot \vec{v}_2 + 8 \hat{n} \cdot \vec{S}_1 \hat{n} \cdot \vec{v}_1 \hat{n} \cdot \vec{v}_2 \vec{S}_1 \cdot \vec{v}_2 + 6 \hat{n} \cdot \vec{v}_1 \vec{S}_1 \cdot \vec{v}_1 \vec{S}_1 \cdot \vec{v}_2 - \\
& 4 \hat{n} \cdot \vec{v}_2 \vec{S}_1 \cdot \vec{v}_1 \vec{S}_1 \cdot \vec{v}_2 - 4 \hat{n} \cdot \vec{v}_1 \vec{S}_1 \cdot \vec{v}_2 \vec{S}_1 \cdot \vec{v}_2 + 2 \hat{n} \cdot \vec{a}_1 \vec{S}_1 \cdot \vec{v}_1 \vec{S}_1 \cdot \vec{v}_2 + 2 \hat{n} \cdot \vec{v}_2 \vec{S}_1 \cdot \vec{S}_1 \vec{v}_1 \cdot \vec{a}_1 - \\
& 4 \hat{n} \cdot \vec{v}_2 \vec{S}_1 \cdot \vec{S}_1 \vec{v}_1 \cdot \vec{v}_1 + 2 \hat{n} \cdot \vec{S}_1 \vec{S}_1 \cdot \vec{v}_2 \vec{v}_1 \cdot \vec{v}_1 - 16 \hat{n} \cdot \vec{v}_1 \vec{S}_1 \cdot \vec{S}_1 \vec{v}_1 \cdot \vec{v}_2 + 20 \hat{n} \cdot \vec{v}_2 \vec{S}_1 \cdot \vec{S}_1 \vec{v}_1 \cdot \vec{v}_2 - \\
& \left. 2 \hat{n} \cdot \vec{a}_1 \vec{S}_1 \cdot \vec{S}_1 \vec{v}_1 \cdot \vec{v}_2 + 6 \hat{n} \cdot \vec{S}_1 \vec{S}_1 \cdot \vec{v}_1 \vec{v}_1 \cdot \vec{v}_2 - 6 \hat{n} \cdot \vec{S}_1 \vec{S}_1 \cdot \vec{v}_2 \vec{v}_1 \cdot \vec{v}_2 + 4 \hat{n} \cdot \vec{v}_1 \vec{S}_1 \cdot \vec{S}_1 \vec{v}_2 \cdot \vec{v}_2 \right) \Big) + \\
& \frac{1}{r^2} \left( 2 \vec{a}_1 \cdot \vec{a}_2 \left( \hat{n} \cdot \vec{S}_1 \right)^2 + 2 \hat{n} \cdot \vec{v}_1 \vec{S}_1 \cdot \vec{a}_2 \hat{n} \cdot \vec{S}_1 + 8 \hat{n} \cdot \vec{v}_1 \vec{S}_1 \cdot \vec{v}_2 \hat{n} \cdot \vec{S}_1 - 8 \hat{n} \cdot \vec{v}_2 \vec{S}_1 \cdot \vec{v}_2 \hat{n} \cdot \vec{S}_1 + \right. \\
& 4 \hat{n} \cdot \vec{S}_1 \vec{v}_1 \cdot \vec{a}_2 \hat{n} \cdot \vec{S}_1 + 8 \left( \vec{S}_1 \cdot \vec{v}_2 \right)^2 + 16 \left( \hat{n} \cdot \vec{v}_2 \right)^2 \vec{S}_1 \cdot \vec{S}_1 - 16 \hat{n} \cdot \vec{v}_1 \hat{n} \cdot \vec{v}_2 \vec{S}_1 \cdot \vec{S}_1 + 16 \hat{n} \cdot \vec{S}_1 \hat{n} \cdot \vec{v}_1 \vec{S}_1 \cdot \vec{v}_2 - \\
& 16 \hat{n} \cdot \vec{S}_1 \hat{n} \cdot \vec{v}_2 \vec{S}_1 \cdot \vec{v}_2 - 8 \vec{S}_1 \cdot \vec{v}_1 \vec{S}_1 \cdot \vec{v}_2 - 4 \hat{n} \cdot \vec{a}_2 \hat{n} \cdot \vec{v}_1 \vec{S}_1 \cdot \vec{S}_1 + 16 \left( \hat{n} \cdot \vec{v}_2 \right)^2 \vec{S}_1 \cdot \vec{S}_1 - \\
& 16 \hat{n} \cdot \vec{v}_1 \hat{n} \cdot \vec{v}_2 \vec{S}_1 \cdot \vec{S}_1 + 2 \hat{n} \cdot \vec{S}_1 \hat{n} \cdot \vec{v}_1 \vec{S}_1 \cdot \vec{a}_2 - 2 \vec{S}_1 \cdot \vec{v}_1 \vec{S}_1 \cdot \vec{a}_2 + 2 \vec{a}_1 \cdot \vec{a}_2 \vec{S}_1 \cdot \vec{S}_1 - 2 \vec{S}_1 \cdot \vec{a}_2 \vec{S}_1 \cdot \vec{v}_1 - \\
& \left. 4 \vec{S}_1 \cdot \vec{v}_2 \vec{S}_1 \cdot \vec{v}_1 + 8 \hat{n} \cdot \vec{S}_1 \hat{n} \cdot \vec{v}_1 \vec{S}_1 \cdot \vec{v}_2 - 8 \hat{n} \cdot \vec{S}_1 \hat{n} \cdot \vec{v}_2 \vec{S}_1 \cdot \vec{v}_2 - 4 \vec{S}_1 \cdot \vec{v}_1 \vec{S}_1 \cdot \vec{v}_2 + 8 \vec{S}_1 \cdot \vec{v}_2 \vec{S}_1 \cdot \vec{v}_2 + \right.
\end{aligned}$$

$$\left. \left( 8 \vec{S}_1 \cdot \vec{S}_1 \vec{v}_1 \cdot \vec{a}_2 + 8 \vec{S}_1 \cdot \vec{S}_1 \vec{v}_1 \cdot \vec{v}_2 + 8 \vec{S}_1 \cdot \vec{S}_1 \vec{v}_1 \cdot \vec{v}_2 - 8 \vec{S}_1 \cdot \vec{S}_1 \vec{v}_2 \cdot \vec{v}_2 - 8 \vec{S}_1 \cdot \vec{S}_1 \vec{v}_2 \cdot \vec{v}_2 \right) \right) m_2 C_{ES^2_1} \}$$

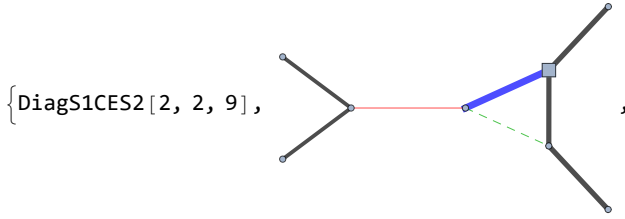

$$\begin{aligned} G^2 \left( \frac{-16 \hat{n} \cdot \vec{a}_1 \vec{S}_1 \cdot \vec{S}_1 + 16 \hat{n} \cdot \vec{S}_1 \vec{S}_1 \cdot \vec{a}_1 + 8 \hat{n} \cdot \vec{S}_1 \vec{S}_1 \cdot \vec{a}_1 - 16 \hat{n} \cdot \vec{a}_1 \vec{S}_1 \cdot \vec{S}_1 + 8 \hat{n} \cdot \vec{S}_1 \vec{S}_1 \cdot \vec{a}_1}{r} + \frac{1}{r^2} \right. \\ \left( -8 \vec{a}_1 \cdot \vec{a}_1 (\hat{n} \cdot \vec{S}_1)^2 - 8 \hat{n} \cdot \vec{v}_1 \vec{S}_1 \cdot \vec{a}_1 \hat{n} \cdot \vec{S}_1 - 8 \hat{n} \cdot \vec{v}_1 \vec{S}_1 \cdot \vec{v}_1 \hat{n} \cdot \vec{S}_1 + 8 \hat{n} \cdot \vec{v}_2 \vec{S}_1 \cdot \vec{v}_1 \hat{n} \cdot \vec{S}_1 - 16 \hat{n} \cdot \vec{S}_1 \vec{v}_1 \cdot \vec{a}_1 \hat{n} \cdot \vec{S}_1 + \right. \\ \left. 8 \left( \vec{S}_1 \cdot \vec{v}_1 \right)^2 + 16 (\hat{n} \cdot \vec{v}_1)^2 \vec{S}_1 \cdot \vec{S}_1 - 16 \hat{n} \cdot \vec{v}_1 \hat{n} \cdot \vec{v}_2 \vec{S}_1 \cdot \vec{S}_1 - 16 \hat{n} \cdot \vec{S}_1 \hat{n} \cdot \vec{v}_1 \vec{S}_1 \cdot \vec{v}_1 + 16 \hat{n} \cdot \vec{S}_1 \hat{n} \cdot \vec{v}_2 \vec{S}_1 \cdot \vec{v}_1 - \right. \\ \left. 8 \vec{S}_1 \cdot \vec{v}_1 \vec{S}_1 \cdot \vec{v}_2 + 16 \hat{n} \cdot \vec{a}_1 \hat{n} \cdot \vec{v}_1 \vec{S}_1 \cdot \vec{S}_1 + 16 (\hat{n} \cdot \vec{v}_1)^2 \vec{S}_1 \cdot \vec{S}_1 - 16 \hat{n} \cdot \vec{v}_1 \hat{n} \cdot \vec{v}_2 \vec{S}_1 \cdot \vec{S}_1 - 8 \hat{n} \cdot \vec{S}_1 \hat{n} \cdot \vec{v}_1 \vec{S}_1 \cdot \vec{a}_1 + \right. \\ \left. 4 \vec{S}_1 \cdot \vec{v}_1 \vec{S}_1 \cdot \vec{a}_1 - 8 \hat{n} \cdot \vec{S}_1 \hat{n} \cdot \vec{v}_1 \vec{S}_1 \cdot \vec{v}_1 + 8 \hat{n} \cdot \vec{S}_1 \hat{n} \cdot \vec{v}_2 \vec{S}_1 \cdot \vec{v}_1 + 4 \vec{S}_1 \cdot \vec{a}_1 \vec{S}_1 \cdot \vec{v}_1 + 8 \vec{S}_1 \cdot \vec{v}_1 \vec{S}_1 \cdot \vec{v}_1 - 4 \vec{S}_1 \cdot \vec{v}_2 \vec{S}_1 \cdot \vec{v}_1 - \right. \\ \left. 4 \vec{S}_1 \cdot \vec{v}_1 \vec{S}_1 \cdot \vec{v}_2 - 8 \vec{S}_1 \cdot \vec{S}_1 \vec{v}_1 \cdot \vec{a}_1 - 8 \vec{S}_1 \cdot \vec{S}_1 \vec{v}_1 \cdot \vec{v}_1 - 8 \vec{S}_1 \cdot \vec{S}_1 \vec{v}_1 \cdot \vec{v}_1 + 8 \vec{S}_1 \cdot \vec{S}_1 \vec{v}_1 \cdot \vec{v}_2 + 8 \vec{S}_1 \cdot \vec{S}_1 \vec{v}_1 \cdot \vec{v}_2 \right) + \\ \frac{1}{r^3} \left( -16 \vec{S}_1 \cdot \vec{S}_1 (\hat{n} \cdot \vec{v}_1)^3 + 8 \hat{n} \cdot \vec{S}_1 \vec{S}_1 \cdot \vec{v}_1 (\hat{n} \cdot \vec{v}_1)^2 + 16 \hat{n} \cdot \vec{v}_2 \vec{S}_1 \cdot \vec{S}_1 (\hat{n} \cdot \vec{v}_1)^2 + 8 \hat{n} \cdot \vec{S}_1 \vec{S}_1 \cdot \vec{v}_1 (\hat{n} \cdot \vec{v}_1)^2 - \right. \\ \left. 8 \hat{n} \cdot \vec{S}_1 \hat{n} \cdot \vec{v}_2 \vec{S}_1 \cdot \vec{v}_1 \hat{n} \cdot \vec{v}_1 - 8 \hat{n} \cdot \vec{S}_1 \hat{n} \cdot \vec{v}_2 \vec{S}_1 \cdot \vec{v}_1 \hat{n} \cdot \vec{v}_1 - 12 \vec{S}_1 \cdot \vec{v}_1 \vec{S}_1 \cdot \vec{v}_1 \hat{n} \cdot \vec{v}_1 + 2 \vec{S}_1 \cdot \vec{v}_2 \vec{S}_1 \cdot \vec{v}_1 \hat{n} \cdot \vec{v}_1 + \right. \\ \left. 2 \vec{S}_1 \cdot \vec{v}_1 \vec{S}_1 \cdot \vec{v}_2 \hat{n} \cdot \vec{v}_1 + 32 (\hat{n} \cdot \vec{S}_1)^2 \vec{v}_1 \cdot \vec{a}_1 \hat{n} \cdot \vec{v}_1 - 4 \vec{S}_1 \cdot \vec{S}_1 \vec{v}_1 \cdot \vec{a}_1 \hat{n} \cdot \vec{v}_1 + 16 \hat{n} \cdot \vec{S}_1 \hat{n} \cdot \vec{S}_1 \vec{v}_1 \cdot \vec{v}_1 \hat{n} \cdot \vec{v}_1 + \right. \\ \left. 20 \vec{S}_1 \cdot \vec{S}_1 \vec{v}_1 \cdot \vec{v}_1 \hat{n} \cdot \vec{v}_1 - 8 \vec{S}_1 \cdot \vec{S}_1 \vec{v}_1 \cdot \vec{v}_2 \hat{n} \cdot \vec{v}_1 - 2 \hat{n} \cdot \vec{a}_1 (\vec{S}_1 \cdot \vec{v}_1)^2 + 8 \hat{n} \cdot \vec{v}_2 \vec{S}_1 \cdot \vec{v}_1 \vec{S}_1 \cdot \vec{v}_1 - 8 (\hat{n} \cdot \vec{S}_1)^2 \hat{n} \cdot \vec{v}_2 \right. \\ \left. \vec{v}_1 \cdot \vec{a}_1 - 4 \hat{n} \cdot \vec{v}_2 \vec{S}_1 \cdot \vec{S}_1 \vec{v}_1 \cdot \vec{a}_1 - 16 \hat{n} \cdot \vec{S}_1 \vec{S}_1 \cdot \vec{v}_1 \vec{v}_1 \cdot \vec{a}_1 + 4 \hat{n} \cdot \vec{S}_1 \vec{S}_1 \cdot \vec{v}_2 \vec{v}_1 \cdot \vec{a}_1 - 16 \hat{n} \cdot \vec{S}_1 \hat{n} \cdot \vec{S}_1 \hat{n} \cdot \vec{v}_2 \vec{v}_1 \cdot \vec{v}_1 - \right. \\ \left. 8 \hat{n} \cdot \vec{S}_1 \vec{S}_1 \cdot \vec{v}_1 \vec{v}_1 \cdot \vec{v}_1 + 4 \hat{n} \cdot \vec{S}_1 \vec{S}_1 \cdot \vec{v}_2 \vec{v}_1 \cdot \vec{v}_1 - 16 \hat{n} \cdot \vec{v}_2 \vec{S}_1 \cdot \vec{S}_1 \vec{v}_1 \cdot \vec{v}_1 + 2 \hat{n} \cdot \vec{a}_1 \vec{S}_1 \cdot \vec{S}_1 \vec{v}_1 \cdot \vec{v}_1 - \right. \\ \left. 8 \hat{n} \cdot \vec{S}_1 \vec{S}_1 \cdot \vec{v}_1 \vec{v}_1 \cdot \vec{v}_1 + 4 \hat{n} \cdot \vec{S}_1 \vec{S}_1 \cdot \vec{v}_2 \vec{v}_1 \cdot \vec{v}_1 + 2 \hat{n} \cdot \vec{S}_1 \vec{S}_1 \cdot \vec{v}_1 \vec{v}_1 \cdot \vec{v}_2 + 2 \hat{n} \cdot \vec{S}_1 \vec{S}_1 \cdot \vec{v}_1 \vec{v}_1 \cdot \vec{v}_2 \right) + \\ \frac{1}{r^4} \left( 4 (\vec{v}_1 \cdot \vec{v}_1)^2 (\hat{n} \cdot \vec{S}_1)^2 - 24 (\hat{n} \cdot \vec{v}_1)^2 \vec{v}_1 \cdot \vec{v}_1 (\hat{n} \cdot \vec{S}_1)^2 + 24 \hat{n} \cdot \vec{v}_1 \hat{n} \cdot \vec{v}_2 \vec{v}_1 \cdot \vec{v}_1 (\hat{n} \cdot \vec{S}_1)^2 - \right. \\ \left. 4 \vec{v}_1 \cdot \vec{v}_1 \vec{v}_1 \cdot \vec{v}_2 (\hat{n} \cdot \vec{S}_1)^2 + 24 \hat{n} \cdot \vec{v}_1 \vec{S}_1 \cdot \vec{v}_1 \vec{v}_1 \cdot \vec{v}_1 \hat{n} \cdot \vec{S}_1 - 16 \hat{n} \cdot \vec{v}_2 \vec{S}_1 \cdot \vec{v}_1 \vec{v}_1 \cdot \vec{v}_1 \hat{n} \cdot \vec{S}_1 - \right. \\ \left. 8 \hat{n} \cdot \vec{v}_1 \vec{S}_1 \cdot \vec{v}_2 \vec{v}_1 \cdot \vec{v}_1 \hat{n} \cdot \vec{S}_1 - 4 (\vec{S}_1 \cdot \vec{v}_1)^2 \vec{v}_1 \cdot \vec{v}_1 + 4 \vec{S}_1 \cdot \vec{v}_1 \vec{S}_1 \cdot \vec{v}_2 \vec{v}_1 \cdot \vec{v}_1 \right) \left. \right) m_2 C_{ES^2_1} \} \end{aligned}$$

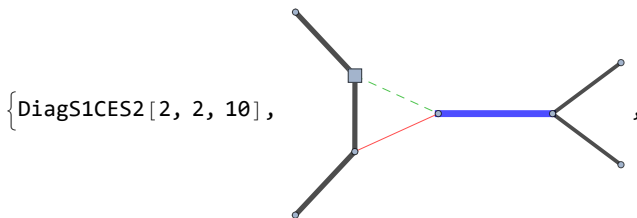

$$G^2 m_2 C_{ES^2_1} \left( \frac{1}{r^3} \left( -4 \vec{a}_1 \cdot \vec{v}_2 (\hat{n} \cdot \vec{S}_1)^2 \hat{n} \cdot \vec{v}_2 + 4 \vec{a}_1 \cdot \vec{v}_2 \hat{n} \cdot \vec{S}_1 \vec{S}_1 \cdot \vec{v}_2 - 8 \vec{v}_1 \cdot \vec{v}_2 \hat{n} \cdot \vec{S}_1 \hat{n} \cdot \vec{S}_1 \hat{n} \cdot \vec{v}_2 + 4 \vec{v}_1 \cdot \vec{v}_2 \hat{n} \cdot \vec{S}_1 \vec{S}_1 \cdot \vec{v}_2 - \right. \right.$$

$$\begin{aligned}
& 2 \hat{n} \cdot \vec{v}_2 \vec{S}_1 \cdot \vec{v}_2 \vec{S}_1 \cdot \vec{v}_1 - 2 \hat{n} \cdot \vec{v}_2 \vec{S}_1 \cdot \vec{v}_1 \vec{S}_1 \cdot \vec{v}_2 + 4 \hat{n} \cdot \vec{v}_1 \vec{S}_1 \cdot \vec{v}_2 \vec{S}_1 \cdot \vec{v}_2 + 4 \vec{S}_1 \cdot \vec{S}_1 \vec{v}_1 \cdot \vec{v}_2 \hat{n} \cdot \vec{v}_2 + \\
& 4 \vec{v}_1 \cdot \vec{v}_2 \hat{n} \cdot \vec{S}_1 \vec{S}_1 \cdot \vec{v}_2 - 4 \vec{S}_1 \cdot \vec{S}_1 \vec{v}_2 \cdot \vec{v}_2 \hat{n} \cdot \vec{v}_1 \Big) + \frac{8 \vec{v}_1 \cdot \vec{v}_2 \hat{n} \cdot \vec{S}_1 \hat{n} \cdot \vec{v}_2 \vec{S}_1 \cdot \vec{v}_1 - 8 \vec{v}_1 \cdot \vec{v}_2 \hat{n} \cdot \vec{S}_1 \hat{n} \cdot \vec{v}_1 \vec{S}_1 \cdot \vec{v}_2}{r^4} + \\
& \frac{1}{r^2} \left( -4 \vec{S}_1 \cdot \vec{S}_1 (\hat{n} \cdot \vec{v}_2)^2 - 4 \vec{S}_1 \cdot \vec{S}_1 (\hat{n} \cdot \vec{v}_1)^2 + 4 \hat{n} \cdot \vec{S}_1 \hat{n} \cdot \vec{v}_2 \vec{S}_1 \cdot \vec{v}_2 + 2 \hat{n} \cdot \vec{S}_1 \hat{n} \cdot \vec{v}_2 \vec{S}_1 \cdot \vec{v}_2 + \right. \\
& \left. 2 \hat{n} \cdot \vec{S}_1 \hat{n} \cdot \vec{v}_2 \vec{S}_1 \cdot \vec{v}_2 - 4 \left( \vec{S}_1 \cdot \vec{v}_2 \right)^2 - 4 \vec{S}_1 \cdot \vec{v}_2 \vec{S}_1 \cdot \vec{v}_2 + 4 \vec{S}_1 \cdot \vec{S}_1 \vec{v}_2 \cdot \vec{v}_2 + 4 \vec{S}_1 \cdot \vec{S}_1 \vec{v}_2 \cdot \vec{v}_2 \right) \Big) \Big\}
\end{aligned}$$

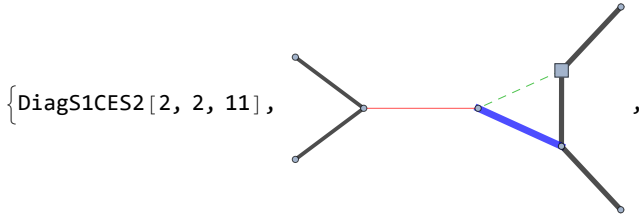

$$\begin{aligned}
& G^2 \left( \frac{1}{r^2} \left( 16 \vec{S}_1 \cdot \vec{S}_1 (\hat{n} \cdot \vec{v}_1)^2 + 16 \vec{S}_1 \cdot \vec{S}_1 (\hat{n} \cdot \vec{v}_1)^2 - 16 \hat{n} \cdot \vec{S}_1 \vec{S}_1 \cdot \vec{v}_1 \hat{n} \cdot \vec{v}_1 - 8 \hat{n} \cdot \vec{S}_1 \vec{S}_1 \cdot \vec{v}_1 \hat{n} \cdot \vec{v}_1 - \right. \right. \\
& \left. 8 \hat{n} \cdot \vec{S}_1 \vec{S}_1 \cdot \vec{v}_1 \hat{n} \cdot \vec{v}_1 + 8 \left( \vec{S}_1 \cdot \vec{v}_1 \right)^2 + 8 \vec{S}_1 \cdot \vec{v}_1 \vec{S}_1 \cdot \vec{v}_1 - 8 \vec{S}_1 \cdot \vec{S}_1 \vec{v}_1 \cdot \vec{v}_1 - 8 \vec{S}_1 \cdot \vec{S}_1 \vec{v}_1 \cdot \vec{v}_1 \right) + \frac{1}{r^3} \\
& \left( -48 \vec{S}_1 \cdot \vec{S}_1 (\hat{n} \cdot \vec{v}_1)^3 + 24 \hat{n} \cdot \vec{S}_1 \vec{S}_1 \cdot \vec{v}_1 (\hat{n} \cdot \vec{v}_1)^2 + 48 \hat{n} \cdot \vec{v}_2 \vec{S}_1 \cdot \vec{S}_1 (\hat{n} \cdot \vec{v}_1)^2 + 24 \hat{n} \cdot \vec{S}_1 \vec{S}_1 \cdot \vec{v}_1 (\hat{n} \cdot \vec{v}_1)^2 - \right. \\
& 24 \hat{n} \cdot \vec{S}_1 \hat{n} \cdot \vec{v}_2 \vec{S}_1 \cdot \vec{v}_1 \hat{n} \cdot \vec{v}_1 - 24 \hat{n} \cdot \vec{S}_1 \hat{n} \cdot \vec{v}_2 \vec{S}_1 \cdot \vec{v}_1 \hat{n} \cdot \vec{v}_1 - 20 \vec{S}_1 \cdot \vec{v}_1 \vec{S}_1 \cdot \vec{v}_1 \hat{n} \cdot \vec{v}_1 + 6 \vec{S}_1 \cdot \vec{v}_2 \vec{S}_1 \cdot \vec{v}_1 \hat{n} \cdot \vec{v}_1 + \\
& 6 \vec{S}_1 \cdot \vec{v}_1 \vec{S}_1 \cdot \vec{v}_2 \hat{n} \cdot \vec{v}_1 + 24 (\hat{n} \cdot \vec{S}_1)^2 \vec{v}_1 \cdot \vec{v}_1 \hat{n} \cdot \vec{v}_1 - 4 \vec{S}_1 \cdot \vec{S}_1 \vec{v}_1 \cdot \vec{v}_1 \hat{n} \cdot \vec{v}_1 + 48 \hat{n} \cdot \vec{S}_1 \hat{n} \cdot \vec{S}_1 \vec{v}_1 \cdot \vec{v}_1 \hat{n} \cdot \vec{v}_1 + \\
& 24 \vec{S}_1 \cdot \vec{S}_1 \vec{v}_1 \cdot \vec{v}_1 \hat{n} \cdot \vec{v}_1 - 24 \vec{S}_1 \cdot \vec{S}_1 \vec{v}_1 \cdot \vec{v}_2 \hat{n} \cdot \vec{v}_1 + 8 \hat{n} \cdot \vec{v}_2 \vec{S}_1 \cdot \vec{v}_1 \vec{S}_1 \cdot \vec{v}_1 - 12 \hat{n} \cdot \vec{S}_1 \vec{S}_1 \cdot \vec{v}_1 \vec{v}_1 \cdot \vec{v}_1 - 18 \hat{n} \cdot \vec{S}_1 \vec{S}_1 \cdot \vec{v}_1 \\
& \left. \vec{v}_1 \cdot \vec{v}_1 - 8 \hat{n} \cdot \vec{v}_2 \vec{S}_1 \cdot \vec{S}_1 \vec{v}_1 \cdot \vec{v}_1 - 18 \hat{n} \cdot \vec{S}_1 \vec{S}_1 \cdot \vec{v}_1 \vec{v}_1 \cdot \vec{v}_1 + 6 \hat{n} \cdot \vec{S}_1 \vec{S}_1 \cdot \vec{v}_1 \vec{v}_1 \cdot \vec{v}_2 + 6 \hat{n} \cdot \vec{S}_1 \vec{S}_1 \cdot \vec{v}_1 \vec{v}_1 \cdot \vec{v}_2 \right) + \\
& \frac{1}{r^4} \left( 20 (\vec{v}_1 \cdot \vec{v}_1)^2 (\hat{n} \cdot \vec{S}_1)^2 - 120 (\hat{n} \cdot \vec{v}_1)^2 \vec{v}_1 \cdot \vec{v}_1 (\hat{n} \cdot \vec{S}_1)^2 + 120 \hat{n} \cdot \vec{v}_1 \hat{n} \cdot \vec{v}_2 \vec{v}_1 \cdot \vec{v}_1 (\hat{n} \cdot \vec{S}_1)^2 - \right. \\
& 20 \vec{v}_1 \cdot \vec{v}_1 \vec{v}_1 \cdot \vec{v}_2 (\hat{n} \cdot \vec{S}_1)^2 + 72 \hat{n} \cdot \vec{v}_1 \vec{S}_1 \cdot \vec{v}_1 \vec{v}_1 \cdot \vec{v}_1 \hat{n} \cdot \vec{S}_1 - 32 \hat{n} \cdot \vec{v}_2 \vec{S}_1 \cdot \vec{v}_1 \vec{v}_1 \cdot \vec{v}_1 \hat{n} \cdot \vec{S}_1 - \\
& 40 \hat{n} \cdot \vec{v}_1 \vec{S}_1 \cdot \vec{v}_2 \vec{v}_1 \cdot \vec{v}_1 \hat{n} \cdot \vec{S}_1 - 4 \vec{S}_1 \cdot \vec{S}_1 (\vec{v}_1 \cdot \vec{v}_1)^2 - 8 (\vec{S}_1 \cdot \vec{v}_1)^2 \vec{v}_1 \cdot \vec{v}_1 + 16 (\hat{n} \cdot \vec{v}_1)^2 \vec{S}_1 \cdot \vec{S}_1 \vec{v}_1 \cdot \vec{v}_1 - \\
& \left. 16 \hat{n} \cdot \vec{v}_1 \hat{n} \cdot \vec{v}_2 \vec{S}_1 \cdot \vec{S}_1 \vec{v}_1 \cdot \vec{v}_1 + 8 \vec{S}_1 \cdot \vec{v}_1 \vec{S}_1 \cdot \vec{v}_2 \vec{v}_1 \cdot \vec{v}_1 + 4 \vec{S}_1 \cdot \vec{S}_1 \vec{v}_1 \cdot \vec{v}_1 \vec{v}_1 \cdot \vec{v}_2 \right) \Big) m_2 C_{ES^2_1} \Big\}
\end{aligned}$$

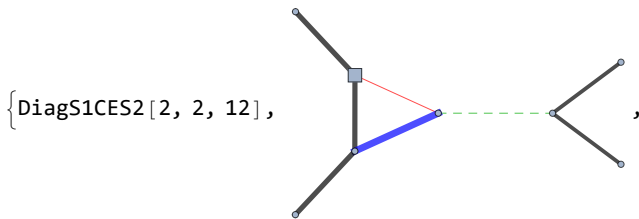

$$\begin{aligned}
& G^2 m_2 C_{ES^2_1} \left( \frac{1}{r^3} \left( -20 \vec{v}_1 \cdot \vec{a}_2 (\hat{n} \cdot \vec{S}_1)^2 \hat{n} \cdot \vec{v}_1 + 8 \vec{v}_1 \cdot \vec{a}_2 \hat{n} \cdot \vec{S}_1 \vec{S}_1 \cdot \vec{v}_1 + 4 \vec{S}_1 \cdot \vec{S}_1 \vec{v}_1 \cdot \vec{a}_2 \hat{n} \cdot \vec{v}_1 - \right. \right. \\
& \left. 48 \vec{v}_1 \cdot \vec{v}_2 \hat{n} \cdot \vec{S}_1 \hat{n} \cdot \vec{S}_1 \hat{n} \cdot \vec{v}_1 + 12 \vec{v}_1 \cdot \vec{v}_2 \hat{n} \cdot \vec{S}_1 \vec{S}_1 \cdot \vec{v}_1 + 8 \vec{S}_1 \cdot \vec{S}_1 \vec{v}_1 \cdot \vec{v}_2 \hat{n} \cdot \vec{v}_1 + 12 \vec{v}_1 \cdot \vec{v}_2 \hat{n} \cdot \vec{S}_1 \vec{S}_1 \cdot \vec{v}_1 \right) + \\
& \frac{1}{r^4} \left( 20 (\vec{v}_1 \cdot \vec{v}_2)^2 (\hat{n} \cdot \vec{S}_1)^2 + 120 \vec{v}_1 \cdot \vec{v}_2 (\hat{n} \cdot \vec{S}_1)^2 (\hat{n} \cdot \vec{v}_1)^2 - 120 \vec{v}_1 \cdot \vec{v}_2 (\hat{n} \cdot \vec{S}_1)^2 \hat{n} \cdot \vec{v}_1 \hat{n} \cdot \vec{v}_2 - \right. \\
& 20 \vec{v}_1 \cdot \vec{v}_1 \vec{v}_1 \cdot \vec{v}_2 (\hat{n} \cdot \vec{S}_1)^2 - 72 \vec{v}_1 \cdot \vec{v}_2 \hat{n} \cdot \vec{S}_1 \hat{n} \cdot \vec{v}_1 \vec{S}_1 \cdot \vec{v}_1 + 32 \vec{v}_1 \cdot \vec{v}_2 \hat{n} \cdot \vec{S}_1 \hat{n} \cdot \vec{v}_2 \vec{S}_1 \cdot \vec{v}_1 + \\
& \left. 40 \vec{v}_1 \cdot \vec{v}_2 \hat{n} \cdot \vec{S}_1 \hat{n} \cdot \vec{v}_1 \vec{S}_1 \cdot \vec{v}_2 - 16 \vec{S}_1 \cdot \vec{S}_1 \vec{v}_1 \cdot \vec{v}_2 (\hat{n} \cdot \vec{v}_1)^2 + 16 \vec{S}_1 \cdot \vec{S}_1 \vec{v}_1 \cdot \vec{v}_2 \hat{n} \cdot \vec{v}_1 \hat{n} \cdot \vec{v}_2 - \right.
\end{aligned}$$





$$\begin{aligned}
& 24 \hat{n} \cdot \vec{S}_1 \vec{S}_1 \cdot \vec{v}_2 \vec{v}_1 \cdot \vec{v}_2 + 8 \hat{n} \cdot \vec{S}_1 \vec{S}_1 \cdot \vec{v}_2 \vec{v}_2 \cdot \vec{v}_2 + 16 \hat{n} \cdot \vec{v}_1 \vec{S}_1 \cdot \vec{S}_1 \vec{v}_2 \cdot \vec{v}_2 + 8 \hat{n} \cdot \vec{S}_1 \vec{S}_1 \cdot \vec{v}_2 \vec{v}_2 \cdot \vec{v}_2 \Big) + \\
& \frac{1}{r^4} \left( 32 (\vec{v}_1 \cdot \vec{v}_2)^2 (\hat{n} \cdot \vec{S}_1)^2 + 192 (\hat{n} \cdot \vec{v}_2)^2 \vec{v}_1 \cdot \vec{v}_2 (\hat{n} \cdot \vec{S}_1)^2 - 192 \hat{n} \cdot \vec{v}_1 \hat{n} \cdot \vec{v}_2 \vec{v}_1 \cdot \vec{v}_2 (\hat{n} \cdot \vec{S}_1)^2 - \right. \\
& 32 \vec{v}_1 \cdot \vec{v}_2 \vec{v}_2 \cdot \vec{v}_2 (\hat{n} \cdot \vec{S}_1)^2 + 64 \hat{n} \cdot \vec{v}_2 \vec{S}_1 \cdot \vec{v}_1 \vec{v}_1 \cdot \vec{v}_2 \hat{n} \cdot \vec{S}_1 + 64 \hat{n} \cdot \vec{v}_1 \vec{S}_1 \cdot \vec{v}_2 \vec{v}_1 \cdot \vec{v}_2 \hat{n} \cdot \vec{S}_1 - \\
& \left. 128 \hat{n} \cdot \vec{v}_2 \vec{S}_1 \cdot \vec{v}_2 \vec{v}_1 \cdot \vec{v}_2 \hat{n} \cdot \vec{S}_1 + 16 (\vec{S}_1 \cdot \vec{v}_2)^2 \vec{v}_1 \cdot \vec{v}_2 - 16 \vec{S}_1 \cdot \vec{v}_1 \vec{S}_1 \cdot \vec{v}_2 \vec{v}_1 \cdot \vec{v}_2 \right) \Big) m_{\text{ES}^2 1}^2 \Big\}
\end{aligned}$$

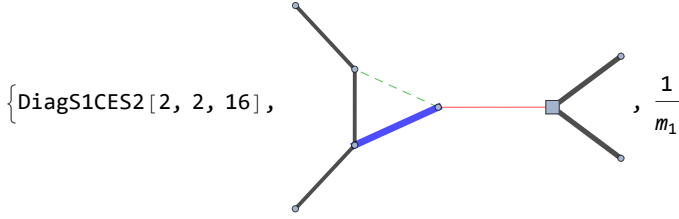

$$\begin{aligned}
& G^2 m_{\text{ES}^2 1}^2 \left( \frac{1}{r^3} \left( -64 \vec{v}_2 \cdot \vec{a}_2 (\hat{n} \cdot \vec{S}_1)^2 \hat{n} \cdot \vec{v}_2 + 32 \vec{v}_2 \cdot \vec{a}_2 \hat{n} \cdot \vec{S}_1 \vec{S}_1 \cdot \vec{v}_2 - 64 \vec{v}_2 \cdot \vec{v}_2 \hat{n} \cdot \vec{S}_1 \hat{n} \cdot \vec{S}_1 \hat{n} \cdot \vec{v}_2 + \right. \right. \\
& 16 \vec{v}_2 \cdot \vec{v}_2 \hat{n} \cdot \vec{S}_1 \vec{S}_1 \cdot \vec{v}_2 + 16 \vec{v}_2 \cdot \vec{v}_2 \hat{n} \cdot \vec{S}_1 \vec{S}_1 \cdot \vec{v}_2 \Big) + \frac{1}{r^4} \left( 32 (\vec{v}_2 \cdot \vec{v}_2)^2 (\hat{n} \cdot \vec{S}_1)^2 - 192 \vec{v}_2 \cdot \vec{v}_2 (\hat{n} \cdot \vec{S}_1)^2 (\hat{n} \cdot \vec{v}_2)^2 + \right. \\
& 192 \vec{v}_2 \cdot \vec{v}_2 (\hat{n} \cdot \vec{S}_1)^2 \hat{n} \cdot \vec{v}_1 \hat{n} \cdot \vec{v}_2 - 32 \vec{v}_1 \cdot \vec{v}_2 \vec{v}_2 \cdot \vec{v}_2 (\hat{n} \cdot \vec{S}_1)^2 - 64 \vec{v}_2 \cdot \vec{v}_2 \hat{n} \cdot \vec{S}_1 \hat{n} \cdot \vec{v}_2 \vec{S}_1 \cdot \vec{v}_1 - \\
& \left. \left. 64 \vec{v}_2 \cdot \vec{v}_2 \hat{n} \cdot \vec{S}_1 \hat{n} \cdot \vec{v}_1 \vec{S}_1 \cdot \vec{v}_2 + 128 \vec{v}_2 \cdot \vec{v}_2 \hat{n} \cdot \vec{S}_1 \hat{n} \cdot \vec{v}_2 \vec{S}_1 \cdot \vec{v}_2 - 16 \vec{v}_2 \cdot \vec{v}_2 (\vec{S}_1 \cdot \vec{v}_2)^2 + 16 \vec{v}_2 \cdot \vec{v}_2 \vec{S}_1 \cdot \vec{v}_1 \vec{S}_1 \cdot \vec{v}_2 \right) \right) \Big\}
\end{aligned}$$

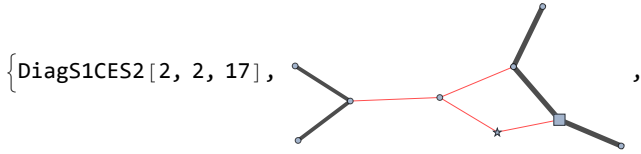

$$\begin{aligned}
& G^2 \left( \frac{1}{r} \left( \frac{1}{6} \hat{n} \cdot \vec{a}_1 \left( \hat{n} \cdot \vec{S}_1 \right)^2 - \frac{2}{3} \hat{n} \cdot \vec{a}_2 \left( \hat{n} \cdot \vec{S}_1 \right)^2 + \frac{1}{3} \vec{S}_1 \cdot \vec{a}_1 \hat{n} \cdot \vec{S}_1 + \frac{2}{3} \vec{S}_1 \cdot \vec{a}_2 \hat{n} \cdot \vec{S}_1 + \right. \right. \\
& \frac{1}{6} \hat{n} \cdot \vec{S}_1 \hat{n} \cdot \vec{a}_1 \hat{n} \cdot \vec{S}_1 - \frac{2}{3} \hat{n} \cdot \vec{S}_1 \hat{n} \cdot \vec{a}_2 \hat{n} \cdot \vec{S}_1 + \frac{7}{6} \hat{n} \cdot \vec{a}_1 \vec{S}_1 \cdot \vec{S}_1 - \frac{8}{3} \hat{n} \cdot \vec{a}_2 \vec{S}_1 \cdot \vec{S}_1 + \frac{1}{6} \hat{n} \cdot \vec{S}_1 \vec{S}_1 \cdot \vec{a}_1 + \\
& \left. \frac{1}{3} \hat{n} \cdot \vec{S}_1 \vec{S}_1 \cdot \vec{a}_2 + \frac{7}{6} \hat{n} \cdot \vec{a}_1 \vec{S}_1 \cdot \vec{S}_1 - \frac{8}{3} \hat{n} \cdot \vec{a}_2 \vec{S}_1 \cdot \vec{S}_1 + \frac{1}{6} \hat{n} \cdot \vec{S}_1 \vec{S}_1 \cdot \vec{a}_1 + \frac{1}{3} \hat{n} \cdot \vec{S}_1 \vec{S}_1 \cdot \vec{a}_2 \right) + \frac{1}{r^2} \\
& \left( -\frac{1}{3} (\hat{n} \cdot \vec{v}_1)^2 \left( \hat{n} \cdot \vec{S}_1 \right)^2 - \frac{8}{3} (\hat{n} \cdot \vec{v}_2)^2 \left( \hat{n} \cdot \vec{S}_1 \right)^2 + \frac{4}{3} \hat{n} \cdot \vec{v}_1 \hat{n} \cdot \vec{v}_2 \left( \hat{n} \cdot \vec{S}_1 \right)^2 + \frac{1}{3} \vec{v}_1 \cdot \vec{v}_1 \left( \hat{n} \cdot \vec{S}_1 \right)^2 - \right. \\
& \frac{1}{3} \vec{v}_1 \cdot \vec{v}_2 \left( \hat{n} \cdot \vec{S}_1 \right)^2 + \frac{2}{3} \vec{v}_2 \cdot \vec{v}_2 \left( \hat{n} \cdot \vec{S}_1 \right)^2 - \frac{2}{3} \hat{n} \cdot \vec{a}_1 \hat{n} \cdot \vec{S}_1 \hat{n} \cdot \vec{v}_1 \hat{n} \cdot \vec{S}_1 + \frac{14}{3} \hat{n} \cdot \vec{a}_2 \hat{n} \cdot \vec{S}_1 \hat{n} \cdot \vec{v}_1 \hat{n} \cdot \vec{S}_1 + \\
& \frac{2}{3} \hat{n} \cdot \vec{a}_1 \hat{n} \cdot \vec{S}_1 \hat{n} \cdot \vec{v}_2 \hat{n} \cdot \vec{S}_1 - \frac{2}{3} \hat{n} \cdot \vec{v}_1 \vec{S}_1 \cdot \vec{v}_1 \hat{n} \cdot \vec{S}_1 + \frac{4}{3} \hat{n} \cdot \vec{v}_2 \vec{S}_1 \cdot \vec{v}_1 \hat{n} \cdot \vec{S}_1 - \frac{2}{3} \hat{n} \cdot \vec{v}_1 \vec{S}_1 \cdot \vec{v}_2 \hat{n} \cdot \vec{S}_1 + \\
& \frac{8}{3} \hat{n} \cdot \vec{v}_2 \vec{S}_1 \cdot \vec{v}_2 \hat{n} \cdot \vec{S}_1 - \frac{1}{6} \hat{n} \cdot \vec{S}_1 \vec{a}_1 \cdot \vec{v}_2 \hat{n} \cdot \vec{S}_1 - \frac{1}{3} \hat{n} \cdot \vec{v}_1 \vec{S}_1 \cdot \vec{a}_1 \hat{n} \cdot \vec{S}_1 + \frac{1}{3} \hat{n} \cdot \vec{v}_2 \vec{S}_1 \cdot \vec{a}_1 \hat{n} \cdot \vec{S}_1 - \frac{7}{6} \hat{n} \cdot \vec{v}_1 \vec{S}_1 \cdot \vec{a}_2 \hat{n} \cdot \vec{S}_1 + \\
& \frac{2}{3} \hat{n} \cdot \vec{a}_1 \vec{S}_1 \cdot \vec{v}_1 \hat{n} \cdot \vec{S}_1 - \frac{5}{3} \hat{n} \cdot \vec{a}_2 \vec{S}_1 \cdot \vec{v}_1 \hat{n} \cdot \vec{S}_1 - \frac{1}{6} \hat{n} \cdot \vec{a}_1 \vec{S}_1 \cdot \vec{v}_2 \hat{n} \cdot \vec{S}_1 - \frac{1}{3} \hat{n} \cdot \vec{S}_1 \vec{v}_1 \cdot \vec{a}_1 \hat{n} \cdot \vec{S}_1 - \frac{7}{6} \hat{n} \cdot \vec{S}_1 \vec{v}_1 \cdot \vec{a}_2 \hat{n} \cdot \vec{S}_1 - \\
& \frac{1}{6} (\hat{n} \cdot \vec{a}_1)^2 (\hat{n} \cdot \vec{S}_1)^2 + \hat{n} \cdot \vec{a}_1 \hat{n} \cdot \vec{a}_2 (\hat{n} \cdot \vec{S}_1)^2 - \frac{1}{3} \hat{n} \cdot \vec{S}_1 \hat{n} \cdot \vec{S}_1 (\hat{n} \cdot \vec{v}_1)^2 - \frac{8}{3} \hat{n} \cdot \vec{S}_1 \hat{n} \cdot \vec{S}_1 (\hat{n} \cdot \vec{v}_2)^2 + \frac{2}{3} \left( \vec{S}_1 \cdot \vec{v}_1 \right)^2 - \\
& \frac{2}{3} \left( \vec{S}_1 \cdot \vec{v}_2 \right)^2 - \frac{1}{6} (\vec{S}_1 \cdot \vec{a}_1)^2 + \frac{4}{3} \hat{n} \cdot \vec{S}_1 \hat{n} \cdot \vec{S}_1 \hat{n} \cdot \vec{v}_1 \hat{n} \cdot \vec{v}_2 - \frac{5}{3} (\hat{n} \cdot \vec{v}_1)^2 \vec{S}_1 \cdot \vec{S}_1 - \frac{16}{3} (\hat{n} \cdot \vec{v}_2)^2 \vec{S}_1 \cdot \vec{S}_1 + \\
& \left. \frac{14}{3} \hat{n} \cdot \vec{v}_1 \hat{n} \cdot \vec{v}_2 \vec{S}_1 \cdot \vec{S}_1 - \frac{1}{3} \hat{n} \cdot \vec{S}_1 \hat{n} \cdot \vec{v}_1 \vec{S}_1 \cdot \vec{a}_1 + \frac{1}{3} \hat{n} \cdot \vec{S}_1 \hat{n} \cdot \vec{v}_2 \vec{S}_1 \cdot \vec{a}_1 - \frac{7}{6} \hat{n} \cdot \vec{S}_1 \hat{n} \cdot \vec{v}_1 \vec{S}_1 \cdot \vec{a}_2 + \right. \\
& \left. \frac{7}{6} \hat{n} \cdot \vec{S}_1 \hat{n} \cdot \vec{v}_2 \vec{S}_1 \cdot \vec{a}_2 \right) \Big\}
\end{aligned}$$



$$\{\text{DiagS1CES2}[2, 2, 18],$$

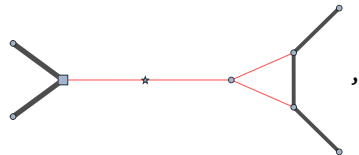

$$\frac{1}{m_1} G^2 \left( \frac{1}{r} \left( -\frac{4}{3} \hat{n} \cdot \vec{a}_2 \left( \hat{n} \cdot \vec{S}_1 \right)^2 + \frac{4}{3} \vec{S}_1 \cdot \vec{a}_2 \hat{n} \cdot \vec{S}_1 - \frac{4}{3} \hat{n} \cdot \vec{S}_1 \hat{n} \cdot \vec{a}_2 \hat{n} \cdot \vec{S}_1 - \right. \right. \\ \left. \left. \frac{4}{3} \hat{n} \cdot \vec{a}_2 \vec{S}_1 \cdot \vec{S}_1 + \frac{2}{3} \hat{n} \cdot \vec{S}_1 \vec{S}_1 \cdot \vec{a}_2 - \frac{4}{3} \hat{n} \cdot \vec{a}_2 \vec{S}_1 \cdot \vec{S}_1 + \frac{2}{3} \hat{n} \cdot \vec{S}_1 \vec{S}_1 \cdot \vec{a}_2 \right) + \frac{1}{r^2} \right.$$



$$\begin{aligned}
& \left( 16 \left( \hat{n} \cdot \vec{S}_1 \right)^2 \hat{n} \cdot \vec{v}_1 \left( \hat{n} \cdot \vec{v}_2 \right)^3 + 4 \hat{n} \cdot \vec{v}_1 \vec{S}_1 \cdot \vec{S}_1 \left( \hat{n} \cdot \vec{v}_2 \right)^3 - 4 \hat{n} \cdot \vec{S}_1 \vec{S}_1 \cdot \vec{v}_1 \left( \hat{n} \cdot \vec{v}_2 \right)^3 - 128 \left( \hat{n} \cdot \vec{S}_1 \right)^2 \left( \hat{n} \cdot \vec{v}_1 \right)^2 \left( \hat{n} \cdot \vec{v}_2 \right)^2 - \right. \\
& \frac{16}{3} \left( \vec{S}_1 \cdot \vec{v}_1 \right)^2 \left( \hat{n} \cdot \vec{v}_2 \right)^2 - 32 \left( \hat{n} \cdot \vec{v}_1 \right)^2 \vec{S}_1 \cdot \vec{S}_1 \left( \hat{n} \cdot \vec{v}_2 \right)^2 + 64 \hat{n} \cdot \vec{S}_1 \hat{n} \cdot \vec{v}_1 \vec{S}_1 \cdot \vec{v}_1 \left( \hat{n} \cdot \vec{v}_2 \right)^2 - \\
& 12 \hat{n} \cdot \vec{S}_1 \hat{n} \cdot \vec{v}_1 \vec{S}_1 \cdot \vec{v}_2 \left( \hat{n} \cdot \vec{v}_2 \right)^2 + 2 \vec{S}_1 \cdot \vec{v}_1 \vec{S}_1 \cdot \vec{v}_2 \left( \hat{n} \cdot \vec{v}_2 \right)^2 + 16 \left( \hat{n} \cdot \vec{S}_1 \right)^2 \vec{v}_1 \cdot \vec{v}_1 \left( \hat{n} \cdot \vec{v}_2 \right)^2 + \\
& \frac{16}{3} \vec{S}_1 \cdot \vec{S}_1 \vec{v}_1 \cdot \vec{v}_1 \left( \hat{n} \cdot \vec{v}_2 \right)^2 - 6 \left( \hat{n} \cdot \vec{S}_1 \right)^2 \vec{v}_1 \cdot \vec{v}_2 \left( \hat{n} \cdot \vec{v}_2 \right)^2 - 2 \vec{S}_1 \cdot \vec{S}_1 \vec{v}_1 \cdot \vec{v}_2 \left( \hat{n} \cdot \vec{v}_2 \right)^2 + \\
& 2 \hat{n} \cdot \vec{v}_1 \left( \vec{S}_1 \cdot \vec{v}_2 \right)^2 \hat{n} \cdot \vec{v}_2 + 64 \hat{n} \cdot \vec{S}_1 \left( \hat{n} \cdot \vec{v}_1 \right)^2 \vec{S}_1 \cdot \vec{v}_2 \hat{n} \cdot \vec{v}_2 - \frac{64}{3} \hat{n} \cdot \vec{v}_1 \vec{S}_1 \cdot \vec{v}_1 \vec{S}_1 \cdot \vec{v}_2 \hat{n} \cdot \vec{v}_2 - \\
& \frac{32}{3} \hat{n} \cdot \vec{S}_1 \vec{S}_1 \cdot \vec{v}_2 \vec{v}_1 \cdot \vec{v}_1 \hat{n} \cdot \vec{v}_2 + 64 \left( \hat{n} \cdot \vec{S}_1 \right)^2 \hat{n} \cdot \vec{v}_1 \vec{v}_1 \cdot \vec{v}_2 \hat{n} \cdot \vec{v}_2 + \frac{64}{3} \hat{n} \cdot \vec{v}_1 \vec{S}_1 \cdot \vec{S}_1 \vec{v}_1 \cdot \vec{v}_2 \hat{n} \cdot \vec{v}_2 - \\
& \frac{64}{3} \hat{n} \cdot \vec{S}_1 \vec{S}_1 \cdot \vec{v}_1 \vec{v}_1 \cdot \vec{v}_2 \hat{n} \cdot \vec{v}_2 + 4 \hat{n} \cdot \vec{S}_1 \vec{S}_1 \cdot \vec{v}_2 \vec{v}_1 \cdot \vec{v}_2 \hat{n} \cdot \vec{v}_2 - 12 \left( \hat{n} \cdot \vec{S}_1 \right)^2 \hat{n} \cdot \vec{v}_1 \vec{v}_2 \cdot \vec{v}_2 \hat{n} \cdot \vec{v}_2 - \\
& 2 \hat{n} \cdot \vec{v}_1 \vec{S}_1 \cdot \vec{S}_1 \vec{v}_2 \cdot \vec{v}_2 \hat{n} \cdot \vec{v}_2 + 4 \hat{n} \cdot \vec{S}_1 \vec{S}_1 \cdot \vec{v}_1 \vec{v}_2 \cdot \vec{v}_2 \hat{n} \cdot \vec{v}_2 - \frac{16}{3} \left( \hat{n} \cdot \vec{v}_1 \right)^2 \left( \vec{S}_1 \cdot \vec{v}_2 \right)^2 - \frac{16}{3} \left( \hat{n} \cdot \vec{S}_1 \right)^2 \left( \vec{v}_1 \cdot \vec{v}_2 \right)^2 - \\
& \frac{8}{3} \vec{S}_1 \cdot \vec{S}_1 \left( \vec{v}_1 \cdot \vec{v}_2 \right)^2 + \frac{4}{3} \left( \vec{S}_1 \cdot \vec{v}_2 \right)^2 \vec{v}_1 \cdot \vec{v}_1 - \frac{1}{2} \left( \vec{S}_1 \cdot \vec{v}_2 \right)^2 \vec{v}_1 \cdot \vec{v}_2 - \frac{64}{3} \hat{n} \cdot \vec{S}_1 \hat{n} \cdot \vec{v}_1 \vec{S}_1 \cdot \vec{v}_2 \vec{v}_1 \cdot \vec{v}_2 + \\
& \frac{16}{3} \vec{S}_1 \cdot \vec{v}_1 \vec{S}_1 \cdot \vec{v}_2 \vec{v}_1 \cdot \vec{v}_2 + 16 \left( \hat{n} \cdot \vec{S}_1 \right)^2 \left( \hat{n} \cdot \vec{v}_1 \right)^2 \vec{v}_2 \cdot \vec{v}_2 + \frac{4}{3} \left( \vec{S}_1 \cdot \vec{v}_1 \right)^2 \vec{v}_2 \cdot \vec{v}_2 + \frac{16}{3} \left( \hat{n} \cdot \vec{v}_1 \right)^2 \vec{S}_1 \cdot \vec{S}_1 \vec{v}_2 \cdot \vec{v}_2 - \\
& \frac{32}{3} \hat{n} \cdot \vec{S}_1 \hat{n} \cdot \vec{v}_1 \vec{S}_1 \cdot \vec{v}_1 \vec{v}_2 \cdot \vec{v}_2 + 4 \hat{n} \cdot \vec{S}_1 \hat{n} \cdot \vec{v}_1 \vec{S}_1 \cdot \vec{v}_2 \vec{v}_2 \cdot \vec{v}_2 - \vec{S}_1 \cdot \vec{v}_1 \vec{S}_1 \cdot \vec{v}_2 \vec{v}_2 \cdot \vec{v}_2 - \frac{8}{3} \left( \hat{n} \cdot \vec{S}_1 \right)^2 \vec{v}_1 \cdot \vec{v}_1 \vec{v}_2 \cdot \vec{v}_2 - \\
& \left. \frac{4}{3} \vec{S}_1 \cdot \vec{S}_1 \vec{v}_1 \cdot \vec{v}_1 \vec{v}_2 \cdot \vec{v}_2 + 2 \left( \hat{n} \cdot \vec{S}_1 \right)^2 \vec{v}_1 \cdot \vec{v}_2 \vec{v}_2 \cdot \vec{v}_2 + \frac{1}{2} \vec{S}_1 \cdot \vec{S}_1 \vec{v}_1 \cdot \vec{v}_2 \vec{v}_2 \cdot \vec{v}_2 \right) \Bigg) m_{\text{ES}}^2 C_{\text{ES}^2 1} \Bigg\}
\end{aligned}$$

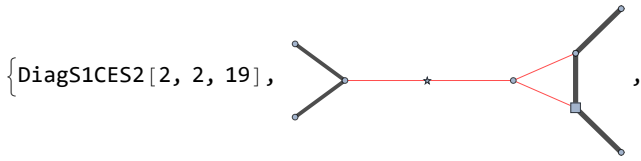

$$\begin{aligned}
& G^2 \left( \frac{- \left( \hat{n} \cdot \vec{a}_2 \right) \left( \hat{n} \cdot \vec{S}_1 \right)^2 + \vec{S}_1 \cdot \vec{a}_2 \hat{n} \cdot \vec{S}_1 - \hat{n} \cdot \vec{S}_1 \hat{n} \cdot \vec{a}_2 \hat{n} \cdot \vec{S}_1 + \frac{1}{2} \hat{n} \cdot \vec{S}_1 \vec{S}_1 \cdot \vec{a}_2 + \frac{1}{2} \hat{n} \cdot \vec{S}_1 \vec{S}_1 \cdot \vec{a}_2}{r} + \frac{1}{r^2} \right. \\
& \left( -4 \left( \hat{n} \cdot \vec{v}_2 \right)^2 \left( \hat{n} \cdot \vec{S}_1 \right)^2 + \frac{2}{3} \hat{n} \cdot \vec{v}_1 \hat{n} \cdot \vec{v}_2 \left( \hat{n} \cdot \vec{S}_1 \right)^2 - \frac{1}{6} \vec{v}_1 \cdot \vec{v}_2 \left( \hat{n} \cdot \vec{S}_1 \right)^2 + \vec{v}_2 \cdot \vec{v}_2 \left( \hat{n} \cdot \vec{S}_1 \right)^2 + 8 \hat{n} \cdot \vec{a}_2 \hat{n} \cdot \vec{S}_1 \hat{n} \cdot \vec{v}_1 \hat{n} \cdot \vec{S}_1 + \right. \\
& \frac{2}{3} \hat{n} \cdot \vec{a}_1 \hat{n} \cdot \vec{S}_1 \hat{n} \cdot \vec{v}_2 \hat{n} \cdot \vec{S}_1 - \frac{4}{3} \hat{n} \cdot \vec{v}_2 \vec{S}_1 \cdot \vec{v}_1 \hat{n} \cdot \vec{S}_1 - \frac{1}{3} \hat{n} \cdot \vec{v}_1 \vec{S}_1 \cdot \vec{v}_2 \hat{n} \cdot \vec{S}_1 + 4 \hat{n} \cdot \vec{v}_2 \vec{S}_1 \cdot \vec{v}_2 \hat{n} \cdot \vec{S}_1 - \\
& \frac{1}{6} \hat{n} \cdot \vec{S}_1 \vec{a}_1 \cdot \vec{v}_2 \hat{n} \cdot \vec{S}_1 - \frac{2}{3} \hat{n} \cdot \vec{v}_2 \vec{S}_1 \cdot \vec{a}_1 \hat{n} \cdot \vec{S}_1 - 2 \hat{n} \cdot \vec{v}_1 \vec{S}_1 \cdot \vec{a}_2 \hat{n} \cdot \vec{S}_1 - 2 \hat{n} \cdot \vec{a}_2 \vec{S}_1 \cdot \vec{v}_1 \hat{n} \cdot \vec{S}_1 - \frac{1}{6} \hat{n} \cdot \vec{a}_1 \vec{S}_1 \cdot \vec{v}_2 \hat{n} \cdot \vec{S}_1 - \\
& 2 \hat{n} \cdot \vec{S}_1 \vec{v}_1 \cdot \vec{a}_2 \hat{n} \cdot \vec{S}_1 + 2 \hat{n} \cdot \vec{a}_1 \hat{n} \cdot \vec{a}_2 \left( \hat{n} \cdot \vec{S}_1 \right)^2 - 4 \hat{n} \cdot \vec{S}_1 \hat{n} \cdot \vec{S}_1 \left( \hat{n} \cdot \vec{v}_2 \right)^2 - \left( \frac{1}{\vec{S}_1 \cdot \vec{v}_2} \right)^2 + \frac{2}{3} \hat{n} \cdot \vec{S}_1 \hat{n} \cdot \vec{S}_1 \hat{n} \cdot \vec{v}_1 \hat{n} \cdot \vec{v}_2 + \\
& \frac{1}{3} \hat{n} \cdot \vec{v}_1 \hat{n} \cdot \vec{v}_2 \vec{S}_1 \cdot \vec{S}_1 - \frac{2}{3} \hat{n} \cdot \vec{S}_1 \hat{n} \cdot \vec{v}_2 \vec{S}_1 \cdot \vec{a}_1 - 2 \hat{n} \cdot \vec{S}_1 \hat{n} \cdot \vec{v}_1 \vec{S}_1 \cdot \vec{a}_2 - 2 \hat{n} \cdot \vec{a}_2 \hat{n} \cdot \vec{S}_1 \vec{S}_1 \cdot \vec{v}_1 - \frac{1}{6} \hat{n} \cdot \vec{a}_1 \hat{n} \cdot \vec{S}_1 \vec{S}_1 \cdot \vec{v}_2 + \\
& \frac{2}{3} \vec{S}_1 \cdot \vec{v}_1 \vec{S}_1 \cdot \vec{v}_2 - \frac{2}{3} \hat{n} \cdot \vec{S}_1 \hat{n} \cdot \vec{v}_2 \vec{S}_1 \cdot \vec{v}_1 - \frac{1}{6} \hat{n} \cdot \vec{S}_1 \hat{n} \cdot \vec{v}_1 \vec{S}_1 \cdot \vec{v}_2 + 2 \hat{n} \cdot \vec{S}_1 \hat{n} \cdot \vec{v}_2 \vec{S}_1 \cdot \vec{v}_2 - \frac{1}{2} \left( \hat{n} \cdot \vec{S}_1 \right)^2 \vec{a}_1 \cdot \vec{a}_2 + \\
& \frac{1}{3} \hat{n} \cdot \vec{a}_1 \hat{n} \cdot \vec{v}_2 \vec{S}_1 \cdot \vec{S}_1 - \frac{1}{6} \vec{a}_1 \cdot \vec{v}_2 \vec{S}_1 \cdot \vec{S}_1 + \frac{1}{3} \hat{n} \cdot \vec{v}_1 \hat{n} \cdot \vec{v}_2 \vec{S}_1 \cdot \vec{S}_1 - \hat{n} \cdot \vec{a}_2 \hat{n} \cdot \vec{S}_1 \vec{S}_1 \cdot \vec{a}_1 + \frac{1}{3} \vec{S}_1 \cdot \vec{v}_2 \vec{S}_1 \cdot \vec{a}_1 - \\
& \hat{n} \cdot \vec{a}_1 \hat{n} \cdot \vec{S}_1 \vec{S}_1 \cdot \vec{a}_2 + \vec{S}_1 \cdot \vec{v}_1 \vec{S}_1 \cdot \vec{a}_2 + \frac{1}{2} \vec{S}_1 \cdot \vec{a}_1 \vec{S}_1 \cdot \vec{a}_2 - \frac{2}{3} \hat{n} \cdot \vec{S}_1 \hat{n} \cdot \vec{v}_2 \vec{S}_1 \cdot \vec{v}_1 + \vec{S}_1 \cdot \vec{a}_2 \vec{S}_1 \cdot \vec{v}_1 + \\
& \left. \frac{1}{3} \vec{S}_1 \cdot \vec{v}_2 \vec{S}_1 \cdot \vec{v}_1 - \frac{1}{6} \hat{n} \cdot \vec{S}_1 \hat{n} \cdot \vec{v}_1 \vec{S}_1 \cdot \vec{v}_2 + 2 \hat{n} \cdot \vec{S}_1 \hat{n} \cdot \vec{v}_2 \vec{S}_1 \cdot \vec{v}_2 + \frac{1}{3} \vec{S}_1 \cdot \vec{a}_1 \vec{S}_1 \cdot \vec{v}_2 + \frac{1}{3} \vec{S}_1 \cdot \vec{v}_1 \vec{S}_1 \cdot \vec{v}_2 - \right.
\end{aligned}$$



$$\left. \frac{5}{4} \left( \hat{n} \cdot \vec{S}_1 \right)^2 \vec{v}_1 \cdot \vec{v}_1 \vec{v}_1 \cdot \vec{v}_2 + \left( \vec{S}_1 \cdot \vec{v}_1 \right)^2 \vec{v}_2 \cdot \vec{v}_2 - 2 \left( \hat{n} \cdot \vec{S}_1 \right)^2 \vec{v}_1 \cdot \vec{v}_1 \vec{v}_2 \cdot \vec{v}_2 \right) m_2 C_{\text{ES}^1} \}$$

$\{\text{DiagS1CES2}[2, 2, 20],$

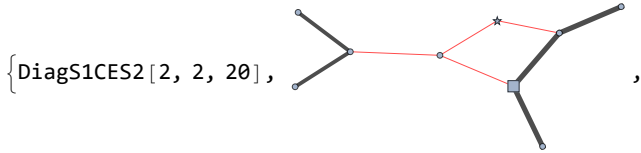

A complex graph structure with black and red edges and various node shapes. It features a central red path with a star node and a square node, connected to other nodes via black edges.

[illegible]





$$\begin{aligned}
& 2 \hat{n} \cdot \vec{S}_1 \vec{S}_1 \cdot \vec{v}_1 \vec{v}_2 \cdot \vec{v}_2 \hat{n} \cdot \vec{v}_1 + 4 (\hat{n} \cdot \vec{v}_2)^2 (\vec{S}_1 \cdot \vec{v}_1)^2 - \frac{3}{4} (\hat{n} \cdot \vec{S}_1)^2 (\vec{v}_1 \cdot \vec{v}_1)^2 + \frac{1}{4} \vec{S}_1 \cdot \vec{S}_1 (\vec{v}_1 \cdot \vec{v}_1)^2 - \\
& 2 (\hat{n} \cdot \vec{S}_1)^2 (\vec{v}_1 \cdot \vec{v}_2)^2 + \vec{S}_1 \cdot \vec{S}_1 (\vec{v}_1 \cdot \vec{v}_2)^2 + 6 (\hat{n} \cdot \vec{S}_1)^2 (\hat{n} \cdot \vec{v}_2)^2 \vec{v}_1 \cdot \vec{v}_1 + \frac{1}{2} (\vec{S}_1 \cdot \vec{v}_2)^2 \vec{v}_1 \cdot \vec{v}_1 - \\
& 2 (\hat{n} \cdot \vec{v}_2)^2 \vec{S}_1 \cdot \vec{S}_1 \vec{v}_1 \cdot \vec{v}_1 - 3 \hat{n} \cdot \vec{S}_1 \hat{n} \cdot \vec{v}_2 \vec{S}_1 \cdot \vec{v}_1 \vec{v}_1 \cdot \vec{v}_1 - 4 \hat{n} \cdot \vec{S}_1 \hat{n} \cdot \vec{v}_2 \vec{S}_1 \cdot \vec{v}_2 \vec{v}_1 \cdot \vec{v}_1 + \frac{3}{4} \vec{S}_1 \cdot \vec{v}_1 \vec{S}_1 \cdot \vec{v}_2 \vec{v}_1 \cdot \vec{v}_1 + \\
& \frac{3}{4} (\vec{S}_1 \cdot \vec{v}_1)^2 \vec{v}_1 \cdot \vec{v}_2 + 4 \hat{n} \cdot \vec{S}_1 \hat{n} \cdot \vec{v}_2 \vec{S}_1 \cdot \vec{v}_1 \vec{v}_1 \cdot \vec{v}_2 - \vec{S}_1 \cdot \vec{v}_1 \vec{S}_1 \cdot \vec{v}_2 \vec{v}_1 \cdot \vec{v}_2 + \frac{15}{8} (\hat{n} \cdot \vec{S}_1)^2 \vec{v}_1 \cdot \vec{v}_1 \vec{v}_1 \cdot \vec{v}_2 - \\
& \frac{9}{8} \vec{S}_1 \cdot \vec{S}_1 \vec{v}_1 \cdot \vec{v}_1 \vec{v}_1 \cdot \vec{v}_2 - (\vec{S}_1 \cdot \vec{v}_1)^2 \vec{v}_2 \cdot \vec{v}_2 - (\hat{n} \cdot \vec{S}_1)^2 \vec{v}_1 \cdot \vec{v}_1 \vec{v}_2 \cdot \vec{v}_2 + \frac{1}{2} \vec{S}_1 \cdot \vec{S}_1 \vec{v}_1 \cdot \vec{v}_1 \vec{v}_2 \cdot \vec{v}_2 \Big) m_2 C_{ES^2_1} \Big\}
\end{aligned}$$

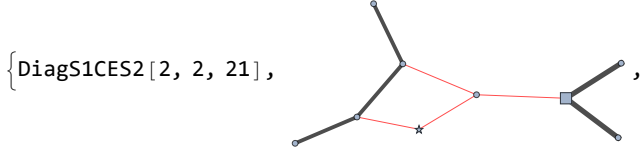

$$\begin{aligned}
& \frac{1}{m_1} G^2 \left( \frac{1}{r} \left( -\frac{4}{3} \hat{n} \cdot \vec{a}_2 \left( \hat{n} \cdot \vec{S}_1 \right)^2 + \frac{4}{3} \vec{S}_1 \cdot \vec{a}_2 \hat{n} \cdot \vec{S}_1 - \frac{4}{3} \hat{n} \cdot \vec{S}_1 \hat{n} \cdot \vec{a}_2 \hat{n} \cdot \vec{S}_1 - \right. \right. \\
& \left. \left. \frac{4}{3} \hat{n} \cdot \vec{a}_2 \vec{S}_1 \cdot \vec{S}_1 + \frac{2}{3} \hat{n} \cdot \vec{S}_1 \vec{S}_1 \cdot \vec{a}_2 - \frac{4}{3} \hat{n} \cdot \vec{a}_2 \vec{S}_1 \cdot \vec{S}_1 + \frac{2}{3} \hat{n} \cdot \vec{S}_1 \vec{S}_1 \cdot \vec{a}_2 \right) + \frac{1}{r^2} \right. \\
& \left( -\frac{16}{3} (\hat{n} \cdot \vec{v}_2)^2 \left( \hat{n} \cdot \vec{S}_1 \right)^2 + \frac{4}{3} \vec{v}_2 \cdot \vec{v}_2 \left( \hat{n} \cdot \vec{S}_1 \right)^2 + \frac{32}{3} \hat{n} \cdot \vec{a}_2 \hat{n} \cdot \vec{S}_1 \hat{n} \cdot \vec{v}_1 \hat{n} \cdot \vec{S}_1 - 8 \hat{n} \cdot \vec{a}_2 \hat{n} \cdot \vec{S}_1 \hat{n} \cdot \vec{v}_2 \hat{n} \cdot \vec{S}_1 + \right. \\
& \frac{16}{3} \hat{n} \cdot \vec{v}_2 \vec{S}_1 \cdot \vec{v}_2 \hat{n} \cdot \vec{S}_1 - \frac{8}{3} \hat{n} \cdot \vec{v}_1 \vec{S}_1 \cdot \vec{a}_2 \hat{n} \cdot \vec{S}_1 + 2 \hat{n} \cdot \vec{v}_2 \vec{S}_1 \cdot \vec{a}_2 \hat{n} \cdot \vec{S}_1 - \frac{8}{3} \hat{n} \cdot \vec{a}_2 \vec{S}_1 \cdot \vec{v}_1 \hat{n} \cdot \vec{S}_1 + 2 \hat{n} \cdot \vec{a}_2 \vec{S}_1 \cdot \vec{v}_2 \hat{n} \cdot \vec{S}_1 - \\
& \frac{8}{3} \hat{n} \cdot \vec{S}_1 \vec{v}_1 \cdot \vec{a}_2 \hat{n} \cdot \vec{S}_1 - 4 \hat{n} \cdot \vec{S}_1 \vec{v}_2 \cdot \vec{a}_2 \hat{n} \cdot \vec{S}_1 - \frac{4}{3} (\hat{n} \cdot \vec{a}_2)^2 (\hat{n} \cdot \vec{S}_1)^2 + \frac{8}{3} \hat{n} \cdot \vec{a}_1 \hat{n} \cdot \vec{a}_2 (\hat{n} \cdot \vec{S}_1)^2 - \\
& \frac{16}{3} \hat{n} \cdot \vec{S}_1 \hat{n} \cdot \vec{S}_1 (\hat{n} \cdot \vec{v}_2)^2 - \frac{4}{3} \left( \vec{S}_1 \cdot \vec{v}_2 \right)^2 - \frac{1}{3} (\vec{S}_1 \cdot \vec{a}_2)^2 - \frac{8}{3} (\hat{n} \cdot \vec{v}_2)^2 \vec{S}_1 \cdot \vec{S}_1 - \frac{8}{3} \hat{n} \cdot \vec{S}_1 \hat{n} \cdot \vec{v}_1 \vec{S}_1 \cdot \vec{a}_2 + \\
& 2 \hat{n} \cdot \vec{S}_1 \hat{n} \cdot \vec{v}_2 \vec{S}_1 \cdot \vec{a}_2 - \frac{8}{3} \hat{n} \cdot \vec{a}_2 \hat{n} \cdot \vec{S}_1 \vec{S}_1 \cdot \vec{v}_1 + 2 \hat{n} \cdot \vec{a}_2 \hat{n} \cdot \vec{S}_1 \vec{S}_1 \cdot \vec{v}_2 + \frac{8}{3} \hat{n} \cdot \vec{S}_1 \hat{n} \cdot \vec{v}_2 \vec{S}_1 \cdot \vec{v}_2 - \\
& \frac{2}{3} (\hat{n} \cdot \vec{S}_1)^2 \vec{a}_1 \cdot \vec{a}_2 - \frac{2}{3} (\hat{n} \cdot \vec{S}_1)^2 \vec{a}_2 \cdot \vec{a}_2 + \frac{16}{3} \hat{n} \cdot \vec{a}_2 \hat{n} \cdot \vec{v}_1 \vec{S}_1 \cdot \vec{S}_1 - 4 \hat{n} \cdot \vec{a}_2 \hat{n} \cdot \vec{v}_2 \vec{S}_1 \cdot \vec{S}_1 - \\
& \frac{8}{3} (\hat{n} \cdot \vec{v}_2)^2 \vec{S}_1 \cdot \vec{S}_1 - \frac{4}{3} \hat{n} \cdot \vec{a}_2 \hat{n} \cdot \vec{S}_1 \vec{S}_1 \cdot \vec{a}_1 - \frac{4}{3} \hat{n} \cdot \vec{a}_1 \hat{n} \cdot \vec{S}_1 \vec{S}_1 \cdot \vec{a}_2 + \frac{4}{3} \hat{n} \cdot \vec{a}_2 \hat{n} \cdot \vec{S}_1 \vec{S}_1 \cdot \vec{a}_2 + \frac{4}{3} \vec{S}_1 \cdot \vec{v}_1 \vec{S}_1 \cdot \vec{a}_2 - \\
& \frac{1}{3} \vec{S}_1 \cdot \vec{v}_2 \vec{S}_1 \cdot \vec{a}_2 + \frac{2}{3} \vec{S}_1 \cdot \vec{a}_1 \vec{S}_1 \cdot \vec{a}_2 - \frac{2}{3} (\hat{n} \cdot \vec{a}_2)^2 \vec{S}_1 \cdot \vec{S}_1 + \frac{4}{3} \hat{n} \cdot \vec{a}_1 \hat{n} \cdot \vec{a}_2 \vec{S}_1 \cdot \vec{S}_1 - \frac{2}{3} \vec{a}_1 \cdot \vec{a}_2 \vec{S}_1 \cdot \vec{S}_1 + \\
& \frac{1}{3} \vec{a}_2 \cdot \vec{a}_2 \vec{S}_1 \cdot \vec{S}_1 + \frac{4}{3} \vec{S}_1 \cdot \vec{a}_2 \vec{S}_1 \cdot \vec{v}_1 + \frac{8}{3} \hat{n} \cdot \vec{S}_1 \hat{n} \cdot \vec{v}_2 \vec{S}_1 \cdot \vec{v}_2 - \vec{S}_1 \cdot \vec{a}_2 \vec{S}_1 \cdot \vec{v}_2 - \frac{4}{3} \vec{S}_1 \cdot \vec{v}_2 \vec{S}_1 \cdot \vec{v}_2 - \\
& \frac{8}{3} \vec{S}_1 \cdot \vec{S}_1 \vec{v}_1 \cdot \vec{a}_2 + 2 \vec{S}_1 \cdot \vec{S}_1 \vec{v}_2 \cdot \vec{a}_2 + \frac{4}{3} \hat{n} \cdot \vec{S}_1 \hat{n} \cdot \vec{S}_1 \vec{v}_2 \cdot \vec{v}_2 + \frac{4}{3} \vec{S}_1 \cdot \vec{S}_1 \vec{v}_2 \cdot \vec{v}_2 + \frac{4}{3} \vec{S}_1 \cdot \vec{S}_1 \vec{v}_2 \cdot \vec{v}_2 \Big) + \frac{1}{r^3} \\
& \left( -20 \hat{n} \cdot \vec{S}_1 \hat{n} \cdot \vec{S}_1 (\hat{n} \cdot \vec{v}_2)^3 - \frac{20}{3} \vec{S}_1 \cdot \vec{S}_1 (\hat{n} \cdot \vec{v}_2)^3 + 16 \hat{n} \cdot \vec{a}_1 (\hat{n} \cdot \vec{S}_1)^2 (\hat{n} \cdot \vec{v}_2)^2 - 8 \hat{n} \cdot \vec{a}_2 (\hat{n} \cdot \vec{S}_1)^2 (\hat{n} \cdot \vec{v}_2)^2 + \right. \\
& 64 \hat{n} \cdot \vec{S}_1 \hat{n} \cdot \vec{S}_1 \hat{n} \cdot \vec{v}_1 (\hat{n} \cdot \vec{v}_2)^2 - \frac{32}{3} \hat{n} \cdot \vec{S}_1 \vec{S}_1 \cdot \vec{v}_1 (\hat{n} \cdot \vec{v}_2)^2 + 10 \hat{n} \cdot \vec{S}_1 \vec{S}_1 \cdot \vec{v}_2 (\hat{n} \cdot \vec{v}_2)^2 + \\
& \frac{64}{3} \hat{n} \cdot \vec{v}_1 \vec{S}_1 \cdot \vec{S}_1 (\hat{n} \cdot \vec{v}_2)^2 - \frac{16}{3} \hat{n} \cdot \vec{S}_1 \vec{S}_1 \cdot \vec{a}_1 (\hat{n} \cdot \vec{v}_2)^2 + \frac{8}{3} \hat{n} \cdot \vec{S}_1 \vec{S}_1 \cdot \vec{a}_2 (\hat{n} \cdot \vec{v}_2)^2 + \\
& \frac{16}{3} \hat{n} \cdot \vec{a}_1 \vec{S}_1 \cdot \vec{S}_1 (\hat{n} \cdot \vec{v}_2)^2 - \frac{8}{3} \hat{n} \cdot \vec{a}_2 \vec{S}_1 \cdot \vec{S}_1 (\hat{n} \cdot \vec{v}_2)^2 - \frac{32}{3} \hat{n} \cdot \vec{S}_1 \vec{S}_1 \cdot \vec{v}_1 (\hat{n} \cdot \vec{v}_2)^2 + \\
& 10 \hat{n} \cdot \vec{S}_1 \vec{S}_1 \cdot \vec{v}_2 (\hat{n} \cdot \vec{v}_2)^2 + 24 \hat{n} \cdot \vec{a}_2 (\hat{n} \cdot \vec{S}_1)^2 \hat{n} \cdot \vec{v}_1 \hat{n} \cdot \vec{v}_2 - \frac{64}{3} \hat{n} \cdot \vec{S}_1 \hat{n} \cdot \vec{v}_1 \vec{S}_1 \cdot \vec{v}_2 \hat{n} \cdot \vec{v}_2 - \\
& \left. \frac{16}{3} (\hat{n} \cdot \vec{S}_1)^2 \vec{a}_1 \cdot \vec{v}_2 \hat{n} \cdot \vec{v}_2 - 8 \hat{n} \cdot \vec{S}_1 \hat{n} \cdot \vec{v}_1 \vec{S}_1 \cdot \vec{a}_2 \hat{n} \cdot \vec{v}_2 + 8 \hat{n} \cdot \vec{a}_2 \hat{n} \cdot \vec{v}_1 \vec{S}_1 \cdot \vec{S}_1 \hat{n} \cdot \vec{v}_2 - \frac{8}{3} \vec{a}_1 \cdot \vec{v}_2 \vec{S}_1 \cdot \vec{S}_1 \hat{n} \cdot \vec{v}_2 - \right.
\end{aligned}$$



$$\frac{8}{3} \left( \hat{n} \cdot \vec{S}_1 \right)^2 \vec{v}_1 \cdot \vec{v}_1 \vec{v}_2 \cdot \vec{v}_2 - \frac{4}{3} \vec{S}_1 \cdot \vec{S}_1 \vec{v}_1 \cdot \vec{v}_1 \vec{v}_2 \cdot \vec{v}_2 + 2 \left( \hat{n} \cdot \vec{S}_1 \right)^2 \vec{v}_1 \cdot \vec{v}_2 \vec{v}_2 \cdot \vec{v}_2 + \frac{5}{2} \vec{S}_1 \cdot \vec{S}_1 \vec{v}_1 \cdot \vec{v}_2 \vec{v}_2 \cdot \vec{v}_2 \right) \Big) m^2 C_{\text{ES}^2_1} \Big\}$$

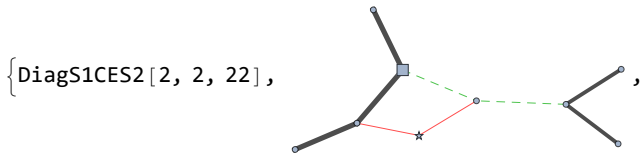

[illegible]

{DiagS1CES2[2, 2, 23],

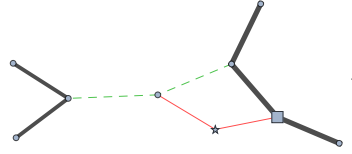

$$\begin{aligned}
 & G^2 \left( \frac{1}{\rho^2} \left( -2 \hat{n} \cdot \vec{S}_1 \hat{n} \cdot \vec{v}_2 \vec{S}_1 \cdot \vec{a}_1 + 2 \hat{n} \cdot \vec{S}_1 \hat{n} \cdot \vec{v}_1 \vec{S}_1 \cdot \vec{a}_2 - 2 \hat{n} \cdot \vec{a}_2 \hat{n} \cdot \vec{S}_1 \vec{S}_1 \cdot \vec{v}_1 + 2 \hat{n} \cdot \vec{a}_1 \hat{n} \cdot \vec{S}_1 \vec{S}_1 \cdot \vec{v}_2 - \right. \right. \\
 & \quad 2 \hat{n} \cdot \vec{S}_1 \hat{n} \cdot \vec{S}_1 \vec{a}_1 \cdot \vec{v}_2 + 6 \vec{a}_1 \cdot \vec{v}_2 \vec{S}_1 \cdot \vec{S}_1 - 2 \hat{n} \cdot \vec{S}_1 \hat{n} \cdot \vec{v}_2 \vec{S}_1 \cdot \vec{a}_1 + 2 \hat{n} \cdot \vec{S}_1 \hat{n} \cdot \vec{v}_1 \vec{S}_1 \cdot \vec{a}_2 - \\
 & \quad \left. \left. 2 \hat{n} \cdot \vec{S}_1 \hat{n} \cdot \vec{a}_2 \vec{S}_1 \cdot \vec{v}_1 + 2 \hat{n} \cdot \vec{S}_1 \hat{n} \cdot \vec{a}_1 \vec{S}_1 \cdot \vec{v}_2 - 2 \hat{n} \cdot \vec{S}_1 \hat{n} \cdot \vec{S}_1 \vec{v}_1 \cdot \vec{a}_2 + 6 \vec{S}_1 \cdot \vec{S}_1 \vec{v}_1 \cdot \vec{a}_2 \right) + \frac{1}{\rho^3} \right. \\
 & \quad \left( 4 \hat{n} \cdot \vec{v}_1 \vec{a}_1 \cdot \vec{v}_2 (\hat{n} \cdot \vec{S}_1)^2 + 2 \hat{n} \cdot \vec{v}_2 \vec{v}_1 \cdot \vec{a}_1 (\hat{n} \cdot \vec{S}_1)^2 + 2 \hat{n} \cdot \vec{v}_1 \vec{v}_1 \cdot \vec{a}_2 (\hat{n} \cdot \vec{S}_1)^2 + 2 \hat{n} \cdot \vec{a}_2 \vec{v}_1 \cdot \vec{v}_1 (\hat{n} \cdot \vec{S}_1)^2 - \right. \\
 & \quad 2 \hat{n} \cdot \vec{a}_1 \vec{v}_1 \cdot \vec{v}_2 (\hat{n} \cdot \vec{S}_1)^2 - 8 (\hat{n} \cdot \vec{v}_2)^2 \vec{S}_1 \cdot \vec{v}_1 \hat{n} \cdot \vec{S}_1 + 4 \hat{n} \cdot \vec{v}_1 \hat{n} \cdot \vec{v}_2 \vec{S}_1 \cdot \vec{v}_1 \hat{n} \cdot \vec{S}_1 - 4 (\hat{n} \cdot \vec{v}_1)^2 \vec{S}_1 \cdot \vec{v}_2 \hat{n} \cdot \vec{S}_1 + \\
 & \quad 8 \hat{n} \cdot \vec{v}_1 \hat{n} \cdot \vec{v}_2 \vec{S}_1 \cdot \vec{v}_2 \hat{n} \cdot \vec{S}_1 + 4 \hat{n} \cdot \vec{v}_1 \hat{n} \cdot \vec{v}_2 \vec{S}_1 \cdot \vec{a}_1 \hat{n} \cdot \vec{S}_1 - 4 (\hat{n} \cdot \vec{v}_1)^2 \vec{S}_1 \cdot \vec{a}_2 \hat{n} \cdot \vec{S}_1 + 4 \hat{n} \cdot \vec{a}_2 \hat{n} \cdot \vec{v}_1 \vec{S}_1 \cdot \vec{v}_1 \hat{n} \cdot \vec{S}_1 - \\
 & \quad 4 \hat{n} \cdot \vec{a}_1 \hat{n} \cdot \vec{v}_1 \vec{S}_1 \cdot \vec{v}_2 \hat{n} \cdot \vec{S}_1 - 4 \hat{n} \cdot \vec{S}_1 \hat{n} \cdot \vec{v}_2 \vec{v}_1 \cdot \vec{v}_1 \hat{n} \cdot \vec{S}_1 + 2 \vec{S}_1 \cdot \vec{v}_2 \vec{v}_1 \cdot \vec{v}_1 \hat{n} \cdot \vec{S}_1 + 4 \hat{n} \cdot \vec{S}_1 \hat{n} \cdot \vec{v}_1 \vec{v}_1 \cdot \vec{v}_2 \hat{n} \cdot \vec{S}_1 - \\
 & \quad 8 \hat{n} \cdot \vec{S}_1 \hat{n} \cdot \vec{v}_2 \vec{v}_1 \cdot \vec{v}_2 \hat{n} \cdot \vec{S}_1 - 4 \vec{S}_1 \cdot \vec{v}_1 \vec{v}_1 \cdot \vec{v}_2 \hat{n} \cdot \vec{S}_1 + 2 \vec{S}_1 \cdot \vec{v}_1 \vec{v}_2 \cdot \vec{v}_2 \hat{n} \cdot \vec{S}_1 - 4 \hat{n} \cdot \vec{v}_1 \vec{a}_1 \cdot \vec{v}_2 \vec{S}_1 \cdot \vec{S}_1 - \\
 & \quad 8 \hat{n} \cdot \vec{S}_1 (\hat{n} \cdot \vec{v}_2)^2 \vec{S}_1 \cdot \vec{v}_1 + 4 \hat{n} \cdot \vec{S}_1 \hat{n} \cdot \vec{v}_1 \hat{n} \cdot \vec{v}_2 \vec{S}_1 \cdot \vec{v}_1 - 4 \hat{n} \cdot \vec{v}_2 \vec{S}_1 \cdot \vec{v}_1 \vec{S}_1 \cdot \vec{v}_1 + 2 \hat{n} \cdot \vec{v}_1 \vec{S}_1 \cdot \vec{v}_2 \vec{S}_1 \cdot \vec{v}_1 + \\
 & \quad 2 \hat{n} \cdot \vec{v}_2 \vec{S}_1 \cdot \vec{v}_2 \vec{S}_1 \cdot \vec{v}_1 - 4 \hat{n} \cdot \vec{S}_1 (\hat{n} \cdot \vec{v}_1)^2 \vec{S}_1 \cdot \vec{v}_2 + 8 \hat{n} \cdot \vec{S}_1 \hat{n} \cdot \vec{v}_1 \hat{n} \cdot \vec{v}_2 \vec{S}_1 \cdot \vec{v}_2 + 2 \hat{n} \cdot \vec{v}_1 \vec{S}_1 \cdot \vec{v}_1 \vec{S}_1 \cdot \vec{v}_2 + \\
 & \quad 2 \hat{n} \cdot \vec{v}_2 \vec{S}_1 \cdot \vec{v}_1 \vec{S}_1 \cdot \vec{v}_2 - 4 \hat{n} \cdot \vec{v}_1 \vec{S}_1 \cdot \vec{v}_2 \vec{S}_1 \cdot \vec{v}_2 - 2 \hat{n} \cdot \vec{v}_2 \vec{S}_1 \cdot \vec{S}_1 \vec{v}_1 \cdot \vec{a}_1 - 2 \hat{n} \cdot \vec{v}_1 \vec{S}_1 \cdot \vec{S}_1 \vec{v}_1 \cdot \vec{a}_2 + \\
 & \quad 4 \hat{n} \cdot \vec{v}_2 \vec{S}_1 \cdot \vec{S}_1 \vec{v}_1 \cdot \vec{v}_1 - 2 \hat{n} \cdot \vec{a}_2 \vec{S}_1 \cdot \vec{S}_1 \vec{v}_1 \cdot \vec{v}_1 + 2 \hat{n} \cdot \vec{S}_1 \vec{S}_1 \cdot \vec{v}_2 \vec{v}_1 \cdot \vec{v}_1 - 8 \hat{n} \cdot \vec{v}_1 \vec{S}_1 \cdot \vec{S}_1 \vec{v}_1 \cdot \vec{v}_2 + \\
 & \quad \left. \left. 12 \hat{n} \cdot \vec{v}_2 \vec{S}_1 \cdot \vec{S}_1 \vec{v}_1 \cdot \vec{v}_2 + 2 \hat{n} \cdot \vec{a}_1 \vec{S}_1 \cdot \vec{S}_1 \vec{v}_1 \cdot \vec{v}_2 - 4 \hat{n} \cdot \vec{S}_1 \vec{S}_1 \cdot \vec{v}_1 \vec{v}_1 \cdot \vec{v}_2 + 2 \hat{n} \cdot \vec{S}_1 \vec{S}_1 \cdot \vec{v}_1 \vec{v}_2 \cdot \vec{v}_2 \right) + \right. \\
 & \quad \left. \frac{1}{\rho^4} \left( 9 \hat{n} \cdot \vec{S}_1 \vec{S}_1 \cdot \vec{v}_2 (\hat{n} \cdot \vec{v}_1)^3 + 4 (\vec{S}_1 \cdot \vec{v}_2)^2 (\hat{n} \cdot \vec{v}_1)^2 - 9 \hat{n} \cdot \vec{S}_1 \hat{n} \cdot \vec{v}_2 \vec{S}_1 \cdot \vec{v}_1 (\hat{n} \cdot \vec{v}_1)^2 - \right. \right. \\
 & \quad 24 \hat{n} \cdot \vec{S}_1 \hat{n} \cdot \vec{v}_2 \vec{S}_1 \cdot \vec{v}_2 (\hat{n} \cdot \vec{v}_1)^2 - 2 \vec{S}_1 \cdot \vec{v}_1 \vec{S}_1 \cdot \vec{v}_2 (\hat{n} \cdot \vec{v}_1)^2 - \frac{9}{2} (\hat{n} \cdot \vec{S}_1)^2 \vec{v}_1 \cdot \vec{v}_2 (\hat{n} \cdot \vec{v}_1)^2 + \\
 & \quad \frac{7}{2} \vec{S}_1 \cdot \vec{S}_1 \vec{v}_1 \cdot \vec{v}_2 (\hat{n} \cdot \vec{v}_1)^2 + 2 \hat{n} \cdot \vec{v}_2 (\vec{S}_1 \cdot \vec{v}_1)^2 \hat{n} \cdot \vec{v}_1 + 24 \hat{n} \cdot \vec{S}_1 (\hat{n} \cdot \vec{v}_2)^2 \vec{S}_1 \cdot \vec{v}_1 \hat{n} \cdot \vec{v}_1 - \\
 & \quad 4 \hat{n} \cdot \vec{v}_2 \vec{S}_1 \cdot \vec{v}_1 \vec{S}_1 \cdot \vec{v}_2 \hat{n} \cdot \vec{v}_1 + 3 (\hat{n} \cdot \vec{S}_1)^2 \hat{n} \cdot \vec{v}_2 \vec{v}_1 \cdot \vec{v}_1 \hat{n} \cdot \vec{v}_1 - \hat{n} \cdot \vec{v}_2 \vec{S}_1 \cdot \vec{S}_1 \vec{v}_1 \cdot \vec{v}_1 \hat{n} \cdot \vec{v}_1 - \\
 & \quad 7 \hat{n} \cdot \vec{S}_1 \vec{S}_1 \cdot \vec{v}_2 \vec{v}_1 \cdot \vec{v}_1 \hat{n} \cdot \vec{v}_1 + 12 (\hat{n} \cdot \vec{S}_1)^2 \hat{n} \cdot \vec{v}_2 \vec{v}_1 \cdot \vec{v}_2 \hat{n} \cdot \vec{v}_1 - 8 \hat{n} \cdot \vec{v}_2 \vec{S}_1 \cdot \vec{S}_1 \vec{v}_1 \cdot \vec{v}_2 \hat{n} \cdot \vec{v}_1 + \\
 & \quad 4 \hat{n} \cdot \vec{S}_1 \vec{S}_1 \cdot \vec{v}_1 \vec{v}_1 \cdot \vec{v}_2 \hat{n} \cdot \vec{v}_1 + 4 \hat{n} \cdot \vec{S}_1 \vec{S}_1 \cdot \vec{v}_2 \vec{v}_1 \cdot \vec{v}_2 \hat{n} \cdot \vec{v}_1 - 4 \hat{n} \cdot \vec{S}_1 \vec{S}_1 \cdot \vec{v}_1 \vec{v}_2 \cdot \vec{v}_2 \hat{n} \cdot \vec{v}_1 - \\
 & \quad 2 (\hat{n} \cdot \vec{S}_1)^2 (\vec{v}_1 \cdot \vec{v}_2)^2 + 2 \vec{S}_1 \cdot \vec{S}_1 (\vec{v}_1 \cdot \vec{v}_2)^2 + 12 (\hat{n} \cdot \vec{S}_1)^2 (\hat{n} \cdot \vec{v}_2)^2 \vec{v}_1 \cdot \vec{v}_1 - 8 (\hat{n} \cdot \vec{v}_2)^2 \vec{S}_1 \cdot \vec{S}_1 \vec{v}_1 \cdot \vec{v}_1 + \\
 & \quad 5 \hat{n} \cdot \vec{S}_1 \hat{n} \cdot \vec{v}_2 \vec{S}_1 \cdot \vec{v}_1 \vec{v}_1 \cdot \vec{v}_1 - 4 \hat{n} \cdot \vec{S}_1 \hat{n} \cdot \vec{v}_2 \vec{S}_1 \cdot \vec{v}_2 \vec{v}_1 \cdot \vec{v}_1 - (\vec{S}_1 \cdot \vec{v}_1)^2 \vec{v}_1 \cdot \vec{v}_2 - 4 \hat{n} \cdot \vec{S}_1 \hat{n} \cdot \vec{v}_2 \vec{S}_1 \cdot \vec{v}_1 \vec{v}_1 \cdot \vec{v}_2 + \\
 & \quad \left. \left. \frac{5}{2} (\hat{n} \cdot \vec{S}_1)^2 \vec{v}_1 \cdot \vec{v}_1 \vec{v}_1 \cdot \vec{v}_2 - \frac{1}{2} \vec{S}_1 \cdot \vec{S}_1 \vec{v}_1 \cdot \vec{v}_1 \vec{v}_1 \cdot \vec{v}_2 - 2 (\hat{n} \cdot \vec{S}_1)^2 \vec{v}_1 \cdot \vec{v}_1 \vec{v}_2 \cdot \vec{v}_2 + 2 \vec{S}_1 \cdot \vec{S}_1 \vec{v}_1 \cdot \vec{v}_1 \vec{v}_2 \cdot \vec{v}_2 \right) \right) m_2 C_{ES^2_1} \}
 \end{aligned}$$

{DiagS1CES2[2, 2, 24],

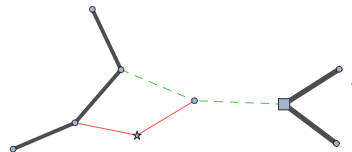

$$\begin{aligned}
 & \frac{1}{m_1} G^2 \left( \frac{1}{\rho^2} \left( 8 \vec{v}_2 \cdot \vec{v}_2 (\hat{n} \cdot \vec{S}_1)^2 - 8 \hat{n} \cdot \vec{v}_2 \vec{S}_1 \cdot \vec{v}_2 \hat{n} \cdot \vec{S}_1 - 4 \hat{n} \cdot \vec{a}_2 \vec{S}_1 \cdot \vec{v}_2 \hat{n} \cdot \vec{S}_1 + \right. \right. \\
 & \quad \left. \left. 8 \hat{n} \cdot \vec{S}_1 \vec{v}_2 \cdot \vec{a}_2 \hat{n} \cdot \vec{S}_1 + 4 \left( \vec{S}_1 \cdot \vec{v}_2 \right)^2 + 8 (\hat{n} \cdot \vec{v}_2)^2 \vec{S}_1 \cdot \vec{S}_1 - 4 \hat{n} \cdot \vec{a}_2 \hat{n} \cdot \vec{S}_1 \vec{S}_1 \cdot \vec{v}_2 - 4 \hat{n} \cdot \vec{S}_1 \hat{n} \cdot \vec{v}_2 \vec{S}_1 \cdot \vec{v}_2 + \right. \right.
 \end{aligned}$$

$$\begin{aligned}
& 8 \hat{n} \cdot \vec{a}_2 \hat{n} \cdot \vec{v}_2 \vec{S}_1 \cdot \vec{S}_1 + 8 (\hat{n} \cdot \vec{v}_2)^2 \vec{S}_1 \cdot \vec{S}_1 + 2 \vec{S}_1 \cdot \vec{v}_2 \vec{S}_1 \cdot \vec{a}_2 - 4 \hat{n} \cdot \vec{S}_1 \hat{n} \cdot \vec{v}_2 \vec{S}_1 \cdot \vec{v}_2 + 2 \vec{S}_1 \cdot \vec{a}_2 \vec{S}_1 \cdot \vec{v}_2 + \\
& 4 \vec{S}_1 \cdot \vec{v}_2 \vec{S}_1 \cdot \vec{v}_2 - 4 \vec{S}_1 \cdot \vec{S}_1 \vec{v}_2 \cdot \vec{a}_2 + 8 \hat{n} \cdot \vec{S}_1 \hat{n} \cdot \vec{S}_1 \vec{v}_2 \cdot \vec{v}_2 - 4 \vec{S}_1 \cdot \vec{S}_1 \vec{v}_2 \cdot \vec{v}_2 - 4 \vec{S}_1 \cdot \vec{S}_1 \vec{v}_2 \cdot \vec{v}_2 \Big) + \frac{1}{r^3} \\
& \left( 24 \vec{S}_1 \cdot \vec{S}_1 (\hat{n} \cdot \vec{v}_2)^3 - 12 \hat{n} \cdot \vec{S}_1 \vec{S}_1 \cdot \vec{v}_2 (\hat{n} \cdot \vec{v}_2)^2 - 32 \hat{n} \cdot \vec{v}_1 \vec{S}_1 \cdot \vec{S}_1 (\hat{n} \cdot \vec{v}_2)^2 - 12 \hat{n} \cdot \vec{S}_1 \vec{S}_1 \cdot \vec{v}_2 (\hat{n} \cdot \vec{v}_2)^2 + \right. \\
& 16 \hat{n} \cdot \vec{S}_1 \hat{n} \cdot \vec{v}_1 \vec{S}_1 \cdot \vec{v}_2 \hat{n} \cdot \vec{v}_2 + 16 (\hat{n} \cdot \vec{S}_1)^2 \vec{a}_1 \cdot \vec{v}_2 \hat{n} \cdot \vec{v}_2 - 4 \vec{S}_1 \cdot \vec{v}_2 \vec{S}_1 \cdot \vec{v}_1 \hat{n} \cdot \vec{v}_2 + \\
& 16 \hat{n} \cdot \vec{S}_1 \hat{n} \cdot \vec{v}_1 \vec{S}_1 \cdot \vec{v}_2 \hat{n} \cdot \vec{v}_2 - 4 \vec{S}_1 \cdot \vec{v}_1 \vec{S}_1 \cdot \vec{v}_2 \hat{n} \cdot \vec{v}_2 + 12 \vec{S}_1 \cdot \vec{v}_2 \vec{S}_1 \cdot \vec{v}_2 \hat{n} \cdot \vec{v}_2 + 32 \hat{n} \cdot \vec{S}_1 \hat{n} \cdot \vec{S}_1 \vec{v}_1 \cdot \vec{v}_2 \hat{n} \cdot \vec{v}_2 + \\
& 16 \vec{S}_1 \cdot \vec{S}_1 \vec{v}_1 \cdot \vec{v}_2 \hat{n} \cdot \vec{v}_2 + 16 \hat{n} \cdot \vec{S}_1 \hat{n} \cdot \vec{S}_1 \vec{v}_2 \cdot \vec{v}_2 \hat{n} \cdot \vec{v}_2 - 12 \vec{S}_1 \cdot \vec{S}_1 \vec{v}_2 \cdot \vec{v}_2 \hat{n} \cdot \vec{v}_2 - \\
& 8 \hat{n} \cdot \vec{v}_1 \vec{S}_1 \cdot \vec{v}_2 \vec{S}_1 \cdot \vec{v}_2 - 8 \hat{n} \cdot \vec{S}_1 \vec{a}_1 \cdot \vec{v}_2 \vec{S}_1 \cdot \vec{v}_2 + 16 \hat{n} \cdot \vec{a}_2 (\hat{n} \cdot \vec{S}_1)^2 \vec{v}_1 \cdot \vec{v}_2 - 12 \hat{n} \cdot \vec{S}_1 \vec{S}_1 \cdot \vec{v}_2 \vec{v}_1 \cdot \vec{v}_2 - \\
& 8 \hat{n} \cdot \vec{S}_1 \vec{S}_1 \cdot \vec{a}_2 \vec{v}_1 \cdot \vec{v}_2 - 12 \hat{n} \cdot \vec{S}_1 \vec{S}_1 \cdot \vec{v}_2 \vec{v}_1 \cdot \vec{v}_2 - 16 (\hat{n} \cdot \vec{S}_1)^2 \hat{n} \cdot \vec{v}_1 \vec{v}_2 \cdot \vec{a}_2 + 8 \hat{n} \cdot \vec{S}_1 \vec{S}_1 \cdot \vec{v}_1 \vec{v}_2 \cdot \vec{a}_2 - \\
& 16 \hat{n} \cdot \vec{a}_1 (\hat{n} \cdot \vec{S}_1)^2 \vec{v}_2 \cdot \vec{v}_2 - 64 \hat{n} \cdot \vec{S}_1 \hat{n} \cdot \vec{S}_1 \hat{n} \cdot \vec{v}_1 \vec{v}_2 \cdot \vec{v}_2 + 16 \hat{n} \cdot \vec{S}_1 \vec{S}_1 \cdot \vec{v}_1 \vec{v}_2 \cdot \vec{v}_2 - 4 \hat{n} \cdot \vec{S}_1 \vec{S}_1 \cdot \vec{v}_2 \vec{v}_2 \cdot \vec{v}_2 + \\
& 8 \hat{n} \cdot \vec{v}_1 \vec{S}_1 \cdot \vec{S}_1 \vec{v}_2 \cdot \vec{v}_2 + 8 \hat{n} \cdot \vec{S}_1 \vec{S}_1 \cdot \vec{a}_1 \vec{v}_2 \cdot \vec{v}_2 + 16 \hat{n} \cdot \vec{S}_1 \vec{S}_1 \cdot \vec{v}_1 \vec{v}_2 \cdot \vec{v}_2 - 4 \hat{n} \cdot \vec{S}_1 \vec{S}_1 \cdot \vec{v}_2 \vec{v}_2 \cdot \vec{v}_2 \Big) + \frac{1}{r^4} \\
& \left( 16 (\vec{v}_1 \cdot \vec{v}_2)^2 (\hat{n} \cdot \vec{S}_1)^2 + 72 (\hat{n} \cdot \vec{v}_2)^2 \vec{v}_1 \cdot \vec{v}_2 (\hat{n} \cdot \vec{S}_1)^2 - 96 \hat{n} \cdot \vec{v}_1 \hat{n} \cdot \vec{v}_2 \vec{v}_1 \cdot \vec{v}_2 (\hat{n} \cdot \vec{S}_1)^2 + 96 (\hat{n} \cdot \vec{v}_1)^2 \right. \\
& \vec{v}_2 \cdot \vec{v}_2 (\hat{n} \cdot \vec{S}_1)^2 - 48 \hat{n} \cdot \vec{v}_1 \hat{n} \cdot \vec{v}_2 \vec{v}_2 \cdot \vec{v}_2 (\hat{n} \cdot \vec{S}_1)^2 - 16 \vec{v}_1 \cdot \vec{v}_1 \vec{v}_2 \cdot \vec{v}_2 (\hat{n} \cdot \vec{S}_1)^2 + 8 \vec{v}_1 \cdot \vec{v}_2 \vec{v}_2 \cdot \vec{v}_2 (\hat{n} \cdot \vec{S}_1)^2 + \\
& 32 \hat{n} \cdot \vec{v}_2 \vec{S}_1 \cdot \vec{v}_1 \vec{v}_1 \cdot \vec{v}_2 \hat{n} \cdot \vec{S}_1 + 32 \hat{n} \cdot \vec{v}_1 \vec{S}_1 \cdot \vec{v}_2 \vec{v}_1 \cdot \vec{v}_2 \hat{n} \cdot \vec{S}_1 - 48 \hat{n} \cdot \vec{v}_2 \vec{S}_1 \cdot \vec{v}_2 \vec{v}_1 \cdot \vec{v}_2 \hat{n} \cdot \vec{S}_1 - \\
& 64 \hat{n} \cdot \vec{v}_1 \vec{S}_1 \cdot \vec{v}_1 \vec{v}_2 \cdot \vec{v}_2 \hat{n} \cdot \vec{S}_1 + 16 \hat{n} \cdot \vec{v}_2 \vec{S}_1 \cdot \vec{v}_1 \vec{v}_2 \cdot \vec{v}_2 \hat{n} \cdot \vec{S}_1 + 16 \hat{n} \cdot \vec{v}_1 \vec{S}_1 \cdot \vec{v}_2 \vec{v}_2 \cdot \vec{v}_2 \hat{n} \cdot \vec{S}_1 + 6 (\vec{S}_1 \cdot \vec{v}_2)^2 \vec{v}_1 \cdot \vec{v}_2 - \\
& 8 \vec{S}_1 \cdot \vec{v}_1 \vec{S}_1 \cdot \vec{v}_2 \vec{v}_1 \cdot \vec{v}_2 + 8 (\vec{S}_1 \cdot \vec{v}_1)^2 \vec{v}_2 \cdot \vec{v}_2 - 4 \vec{S}_1 \cdot \vec{v}_1 \vec{S}_1 \cdot \vec{v}_2 \vec{v}_2 \cdot \vec{v}_2 - 6 \vec{S}_1 \cdot \vec{S}_1 \vec{v}_1 \cdot \vec{v}_2 \vec{v}_2 \cdot \vec{v}_2 \Big) m_2^2 C_{ES^2_1} \Big\}
\end{aligned}$$

{DiagS1CES2[2, 2, 25],

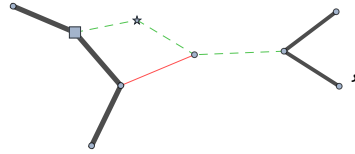

$$\begin{aligned}
& G^2 \left( \frac{12 \hat{n} \cdot \vec{a}_2 \vec{S}_1 \cdot \vec{S}_1 - 4 \hat{n} \cdot \vec{S}_1 \vec{S}_1 \cdot \vec{a}_2 - 2 \hat{n} \cdot \vec{S}_1 \vec{S}_1 \cdot \vec{a}_2 + 12 \hat{n} \cdot \vec{a}_2 \vec{S}_1 \cdot \vec{S}_1 - 2 \hat{n} \cdot \vec{S}_1 \vec{S}_1 \cdot \vec{a}_2}{r} + \frac{1}{r^2} \right. \\
& \left( 2 \vec{v}_1 \cdot \vec{v}_2 (\hat{n} \cdot \vec{S}_1)^2 - 2 \hat{n} \cdot \vec{v}_2 \vec{S}_1 \cdot \vec{v}_1 \hat{n} \cdot \vec{S}_1 - 8 \hat{n} \cdot \vec{v}_2 \vec{S}_1 \cdot \vec{v}_2 \hat{n} \cdot \vec{S}_1 + 2 \hat{n} \cdot \vec{v}_1 \vec{S}_1 \cdot \vec{a}_2 \hat{n} \cdot \vec{S}_1 + 3 \hat{n} \cdot \vec{a}_2 \vec{S}_1 \cdot \vec{v}_1 \hat{n} \cdot \vec{S}_1 + \right. \\
& 8 \hat{n} \cdot \vec{S}_1 \vec{v}_1 \cdot \vec{a}_2 \hat{n} \cdot \vec{S}_1 + 4 (\vec{S}_1 \cdot \vec{v}_2)^2 + 24 (\hat{n} \cdot \vec{v}_2)^2 \vec{S}_1 \cdot \vec{S}_1 - 10 \hat{n} \cdot \vec{v}_1 \hat{n} \cdot \vec{v}_2 \vec{S}_1 \cdot \vec{S}_1 + 2 \hat{n} \cdot \vec{S}_1 \hat{n} \cdot \vec{v}_1 \vec{S}_1 \cdot \vec{a}_2 + \\
& 3 \hat{n} \cdot \vec{a}_2 \hat{n} \cdot \vec{S}_1 \vec{S}_1 \cdot \vec{v}_1 + 2 \vec{S}_1 \cdot \vec{v}_1 \vec{S}_1 \cdot \vec{v}_2 - \hat{n} \cdot \vec{S}_1 \hat{n} \cdot \vec{v}_2 \vec{S}_1 \cdot \vec{v}_1 - 4 \hat{n} \cdot \vec{S}_1 \hat{n} \cdot \vec{v}_2 \vec{S}_1 \cdot \vec{v}_2 + 5 (\hat{n} \cdot \vec{S}_1)^2 \vec{a}_1 \cdot \vec{a}_2 - \\
& 14 \hat{n} \cdot \vec{a}_2 \hat{n} \cdot \vec{v}_1 \vec{S}_1 \cdot \vec{S}_1 + 24 (\hat{n} \cdot \vec{v}_2)^2 \vec{S}_1 \cdot \vec{S}_1 - 10 \hat{n} \cdot \vec{v}_1 \hat{n} \cdot \vec{v}_2 \vec{S}_1 \cdot \vec{S}_1 + 2 \hat{n} \cdot \vec{a}_2 \hat{n} \cdot \vec{S}_1 \vec{S}_1 \cdot \vec{a}_1 - \\
& 2 \hat{n} \cdot \vec{a}_1 \hat{n} \cdot \vec{S}_1 \vec{S}_1 \cdot \vec{a}_2 - 3 \vec{S}_1 \cdot \vec{v}_1 \vec{S}_1 \cdot \vec{a}_2 + \vec{a}_1 \cdot \vec{a}_2 \vec{S}_1 \cdot \vec{S}_1 - \hat{n} \cdot \vec{S}_1 \hat{n} \cdot \vec{v}_2 \vec{S}_1 \cdot \vec{v}_1 - 3 \vec{S}_1 \cdot \vec{a}_2 \vec{S}_1 \cdot \vec{v}_1 + \\
& \vec{S}_1 \cdot \vec{v}_2 \vec{S}_1 \cdot \vec{v}_1 - 4 \hat{n} \cdot \vec{S}_1 \hat{n} \cdot \vec{v}_2 \vec{S}_1 \cdot \vec{v}_2 + \vec{S}_1 \cdot \vec{v}_1 \vec{S}_1 \cdot \vec{v}_2 + 4 \vec{S}_1 \cdot \vec{v}_2 \vec{S}_1 \cdot \vec{v}_2 + 10 \vec{S}_1 \cdot \vec{S}_1 \vec{v}_1 \cdot \vec{a}_2 + \\
& 2 \hat{n} \cdot \vec{S}_1 \hat{n} \cdot \vec{S}_1 \vec{v}_1 \cdot \vec{v}_2 + 4 \vec{S}_1 \cdot \vec{S}_1 \vec{v}_1 \cdot \vec{v}_2 + 4 \vec{S}_1 \cdot \vec{S}_1 \vec{v}_1 \cdot \vec{v}_2 - 12 \vec{S}_1 \cdot \vec{S}_1 \vec{v}_2 \cdot \vec{v}_2 - 12 \vec{S}_1 \cdot \vec{S}_1 \vec{v}_2 \cdot \vec{v}_2 \Big) + \frac{1}{r^3} \\
& \left( -4 \hat{n} \cdot \vec{v}_1 \vec{a}_1 \cdot \vec{v}_2 (\hat{n} \cdot \vec{S}_1)^2 + 20 \hat{n} \cdot \vec{v}_2 \vec{a}_1 \cdot \vec{v}_2 (\hat{n} \cdot \vec{S}_1)^2 + 2 \hat{n} \cdot \vec{v}_2 \vec{v}_1 \cdot \vec{a}_1 (\hat{n} \cdot \vec{S}_1)^2 - 14 \hat{n} \cdot \vec{v}_1 \vec{v}_1 \cdot \vec{a}_2 (\hat{n} \cdot \vec{S}_1)^2 - \right. \\
& 2 \hat{n} \cdot \vec{a}_2 \vec{v}_1 \cdot \vec{v}_1 (\hat{n} \cdot \vec{S}_1)^2 - 2 \hat{n} \cdot \vec{a}_1 \vec{v}_1 \cdot \vec{v}_2 (\hat{n} \cdot \vec{S}_1)^2 + 12 (\hat{n} \cdot \vec{v}_2)^2 \vec{S}_1 \cdot \vec{v}_1 \hat{n} \cdot \vec{S}_1 - 4 \hat{n} \cdot \vec{v}_1 \hat{n} \cdot \vec{v}_2 \vec{S}_1 \cdot \vec{v}_1 \hat{n} \cdot \vec{S}_1 + \\
& 2 (\hat{n} \cdot \vec{v}_1)^2 \vec{S}_1 \cdot \vec{v}_2 \hat{n} \cdot \vec{S}_1 + 8 \hat{n} \cdot \vec{v}_1 \hat{n} \cdot \vec{v}_2 \vec{S}_1 \cdot \vec{v}_2 \hat{n} \cdot \vec{S}_1 + 8 (\hat{n} \cdot \vec{v}_2)^2 \vec{S}_1 \cdot \vec{a}_1 \hat{n} \cdot \vec{S}_1 -
\end{aligned}$$



$$\begin{aligned}
& 8 \hat{n} \cdot \vec{S}_1 \hat{n} \cdot \vec{v}_1 \hat{n} \cdot \vec{v}_2 \vec{S}_1 \cdot \vec{v}_2 - 2 \hat{n} \cdot \vec{v}_2 \vec{S}_1 \cdot \vec{v}_1 \vec{S}_1 \cdot \vec{v}_2 + 4 \hat{n} \cdot \vec{v}_1 \vec{S}_1 \cdot \vec{v}_2 \vec{S}_1 \cdot \vec{v}_2 - 2 \hat{n} \cdot \vec{v}_2 \vec{S}_1 \cdot \vec{a}_1 \vec{S}_1 \cdot \vec{v}_2 + \\
& 2 \hat{n} \cdot \vec{v}_1 \vec{S}_1 \cdot \vec{S}_1 \vec{v}_1 \cdot \vec{a}_2 - 4 \hat{n} \cdot \vec{v}_2 \vec{S}_1 \cdot \vec{S}_1 \vec{v}_1 \cdot \vec{v}_2 - 4 \hat{n} \cdot \vec{S}_1 \vec{S}_1 \cdot \vec{v}_2 \vec{v}_1 \cdot \vec{v}_2 - 2 \hat{n} \cdot \vec{S}_1 \vec{S}_1 \cdot \vec{v}_1 \vec{v}_2 \cdot \vec{v}_2 \Big) + \frac{1}{r^4} \\
& \left( 12 (\vec{v}_1 \cdot \vec{v}_2)^2 (\hat{n} \cdot \vec{S}_1)^2 - 72 \hat{n} \cdot \vec{v}_1 \hat{n} \cdot \vec{v}_2 \vec{v}_1 \cdot \vec{v}_2 (\hat{n} \cdot \vec{S}_1)^2 - 48 \hat{n} \cdot \vec{v}_1 (\hat{n} \cdot \vec{v}_2)^2 \vec{S}_1 \cdot \vec{v}_1 \hat{n} \cdot \vec{S}_1 + 48 (\hat{n} \cdot \vec{v}_1)^2 \right. \\
& \hat{n} \cdot \vec{v}_2 \vec{S}_1 \cdot \vec{v}_2 \hat{n} \cdot \vec{S}_1 - 8 \hat{n} \cdot \vec{v}_2 \vec{S}_1 \cdot \vec{v}_2 \vec{v}_1 \cdot \vec{v}_1 \hat{n} \cdot \vec{S}_1 + 40 \hat{n} \cdot \vec{v}_2 \vec{S}_1 \cdot \vec{v}_1 \vec{v}_1 \cdot \vec{v}_2 \hat{n} \cdot \vec{S}_1 + 8 \hat{n} \cdot \vec{v}_1 \vec{S}_1 \cdot \vec{v}_2 \vec{v}_1 \cdot \vec{v}_2 \hat{n} \cdot \vec{S}_1 + \\
& 8 \hat{n} \cdot \vec{v}_1 \vec{S}_1 \cdot \vec{v}_1 \vec{v}_2 \cdot \vec{v}_2 \hat{n} \cdot \vec{S}_1 + 8 (\hat{n} \cdot \vec{v}_2)^2 (\vec{S}_1 \cdot \vec{v}_1)^2 - 8 (\hat{n} \cdot \vec{v}_1)^2 (\vec{S}_1 \cdot \vec{v}_2)^2 - 2 \vec{S}_1 \cdot \vec{S}_1 (\vec{v}_1 \cdot \vec{v}_2)^2 + \\
& \left. 2 (\vec{S}_1 \cdot \vec{v}_2)^2 \vec{v}_1 \cdot \vec{v}_1 + 8 \hat{n} \cdot \vec{v}_1 \hat{n} \cdot \vec{v}_2 \vec{S}_1 \cdot \vec{S}_1 \vec{v}_1 \cdot \vec{v}_2 - 6 \vec{S}_1 \cdot \vec{v}_1 \vec{S}_1 \cdot \vec{v}_2 \vec{v}_1 \cdot \vec{v}_2 - 2 (\vec{S}_1 \cdot \vec{v}_1)^2 \vec{v}_2 \cdot \vec{v}_2 \right) m_2 C_{ES^2 1} \Big\}
\end{aligned}$$

$$\left\{ \text{DiagS1CES2}[2, 2, 27], \right.$$
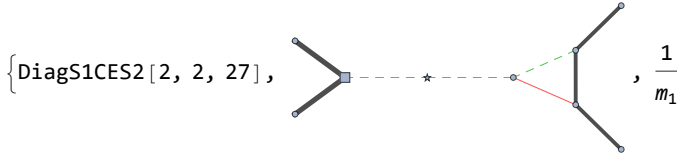

$$, \frac{1}{m_1}$$

$$\begin{aligned}
& G^2 \left( \frac{8 \hat{n} \cdot \vec{a}_2 \vec{S}_1 \cdot \vec{S}_1 - 8 \hat{n} \cdot \vec{S}_1 \vec{S}_1 \cdot \vec{a}_2 - 4 \hat{n} \cdot \vec{S}_1 \vec{S}_1 \cdot \vec{a}_2 + 8 \hat{n} \cdot \vec{a}_2 \vec{S}_1 \cdot \vec{S}_1 - 4 \hat{n} \cdot \vec{S}_1 \vec{S}_1 \cdot \vec{a}_2}{r} + \right. \\
& \frac{1}{r^4} \left( 32 (\vec{v}_1 \cdot \vec{v}_2)^2 (\hat{n} \cdot \vec{S}_1)^2 - 192 \hat{n} \cdot \vec{v}_1 \hat{n} \cdot \vec{v}_2 \vec{v}_1 \cdot \vec{v}_2 (\hat{n} \cdot \vec{S}_1)^2 + \right. \\
& 64 \hat{n} \cdot \vec{v}_2 \vec{S}_1 \cdot \vec{v}_1 \vec{v}_1 \cdot \vec{v}_2 \hat{n} \cdot \vec{S}_1 + 64 \hat{n} \cdot \vec{v}_1 \vec{S}_1 \cdot \vec{v}_2 \vec{v}_1 \cdot \vec{v}_2 \hat{n} \cdot \vec{S}_1 - 16 \vec{S}_1 \cdot \vec{v}_1 \vec{S}_1 \cdot \vec{v}_2 \vec{v}_1 \cdot \vec{v}_2 \Big) + \\
& \frac{1}{r^3} \left( 32 \hat{n} \cdot \vec{v}_2 \vec{a}_1 \cdot \vec{v}_2 (\hat{n} \cdot \vec{S}_1)^2 - 32 \hat{n} \cdot \vec{v}_1 \vec{v}_1 \cdot \vec{a}_2 (\hat{n} \cdot \vec{S}_1)^2 + 32 \hat{n} \cdot \vec{v}_1 \hat{n} \cdot \vec{v}_2 \vec{S}_1 \cdot \vec{v}_2 \hat{n} \cdot \vec{S}_1 - \right. \\
& 16 \vec{a}_1 \cdot \vec{v}_2 \vec{S}_1 \cdot \vec{v}_2 \hat{n} \cdot \vec{S}_1 + 16 \vec{S}_1 \cdot \vec{v}_1 \vec{v}_1 \cdot \vec{a}_2 \hat{n} \cdot \vec{S}_1 + 64 \hat{n} \cdot \vec{S}_1 \hat{n} \cdot \vec{v}_2 \vec{v}_1 \cdot \vec{v}_2 \hat{n} \cdot \vec{S}_1 - 24 \vec{S}_1 \cdot \vec{v}_2 \vec{v}_1 \cdot \vec{v}_2 \hat{n} \cdot \vec{S}_1 - \\
& 64 \hat{n} \cdot \vec{v}_1 (\hat{n} \cdot \vec{v}_2)^2 \vec{S}_1 \cdot \vec{S}_1 - 8 \hat{n} \cdot \vec{v}_2 \vec{S}_1 \cdot \vec{v}_2 \vec{S}_1 \cdot \vec{v}_1 + 32 \hat{n} \cdot \vec{S}_1 \hat{n} \cdot \vec{v}_1 \hat{n} \cdot \vec{v}_2 \vec{S}_1 \cdot \vec{v}_2 - 8 \hat{n} \cdot \vec{v}_2 \vec{S}_1 \cdot \vec{v}_1 \vec{S}_1 \cdot \vec{v}_2 - \\
& 16 \hat{n} \cdot \vec{v}_1 \vec{S}_1 \cdot \vec{v}_2 \vec{S}_1 \cdot \vec{v}_2 + 32 \hat{n} \cdot \vec{v}_2 \vec{S}_1 \cdot \vec{S}_1 \vec{v}_1 \cdot \vec{v}_2 - 24 \hat{n} \cdot \vec{S}_1 \vec{S}_1 \cdot \vec{v}_2 \vec{v}_1 \cdot \vec{v}_2 + 16 \hat{n} \cdot \vec{v}_1 \vec{S}_1 \cdot \vec{S}_1 \vec{v}_2 \cdot \vec{v}_2 \Big) + \\
& \frac{1}{r^2} \left( 8 \vec{a}_1 \cdot \vec{a}_2 (\hat{n} \cdot \vec{S}_1)^2 + 8 \hat{n} \cdot \vec{v}_1 \vec{S}_1 \cdot \vec{a}_2 \hat{n} \cdot \vec{S}_1 - 8 \hat{n} \cdot \vec{v}_2 \vec{S}_1 \cdot \vec{v}_2 \hat{n} \cdot \vec{S}_1 + 16 \hat{n} \cdot \vec{S}_1 \vec{v}_1 \cdot \vec{a}_2 \hat{n} \cdot \vec{S}_1 + \right. \\
& 8 \left( \frac{1}{\vec{S}_1 \cdot \vec{v}_2} \right)^2 + 16 (\hat{n} \cdot \vec{v}_2)^2 \frac{1}{\vec{S}_1 \cdot \vec{S}_1} - 16 \hat{n} \cdot \vec{S}_1 \hat{n} \cdot \vec{v}_2 \vec{S}_1 \cdot \vec{v}_2 - 16 \hat{n} \cdot \vec{a}_2 \hat{n} \cdot \vec{v}_1 \vec{S}_1 \cdot \vec{S}_1 + \\
& 16 (\hat{n} \cdot \vec{v}_2)^2 \vec{S}_1 \cdot \vec{S}_1 + 8 \hat{n} \cdot \vec{S}_1 \hat{n} \cdot \vec{v}_1 \vec{S}_1 \cdot \vec{a}_2 - 4 \vec{S}_1 \cdot \vec{v}_1 \vec{S}_1 \cdot \vec{a}_2 - 4 \vec{S}_1 \cdot \vec{a}_2 \vec{S}_1 \cdot \vec{v}_1 - 8 \hat{n} \cdot \vec{S}_1 \hat{n} \cdot \vec{v}_2 \vec{S}_1 \cdot \vec{v}_2 + \\
& \left. 8 \vec{S}_1 \cdot \vec{v}_2 \vec{S}_1 \cdot \vec{v}_2 + 8 \vec{S}_1 \cdot \vec{S}_1 \vec{v}_1 \cdot \vec{a}_2 - 8 \vec{S}_1 \cdot \vec{S}_1 \vec{v}_2 \cdot \vec{v}_2 - 8 \vec{S}_1 \cdot \vec{S}_1 \vec{v}_2 \cdot \vec{v}_2 \right) \Big\} m_2^2 C_{ES^2 1}
\end{aligned}$$

$$\left\{ \text{DiagS1CES2}[2, 2, 28], \right.$$
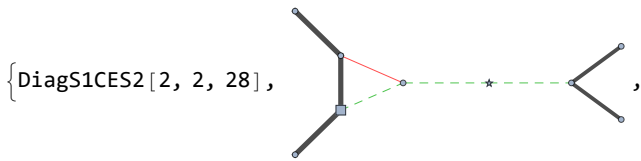

$$,$$

$$\begin{aligned}
& G^2 \left( \frac{2 \hat{n} \cdot \vec{a}_2 \vec{S}_1 \cdot \vec{S}_1 - 6 \hat{n} \cdot \vec{S}_1 \vec{S}_1 \cdot \vec{a}_2 - 3 \hat{n} \cdot \vec{S}_1 \vec{S}_1 \cdot \vec{a}_2 + 2 \hat{n} \cdot \vec{a}_2 \vec{S}_1 \cdot \vec{S}_1 - 3 \hat{n} \cdot \vec{S}_1 \vec{S}_1 \cdot \vec{a}_2}{r} + \frac{1}{r^2} \right. \\
& \left( 3 \vec{a}_1 \cdot \vec{a}_2 (\hat{n} \cdot \vec{S}_1)^2 + 8 \hat{n} \cdot \vec{v}_1 \vec{S}_1 \cdot \vec{a}_2 \hat{n} \cdot \vec{S}_1 - 2 \hat{n} \cdot \vec{a}_2 \vec{S}_1 \cdot \vec{v}_1 \hat{n} \cdot \vec{S}_1 - 6 \hat{n} \cdot \vec{v}_2 \vec{S}_1 \cdot \vec{v}_2 \hat{n} \cdot \vec{S}_1 - 2 \hat{n} \cdot \vec{a}_2 \vec{S}_1 \cdot \vec{a}_1 \hat{n} \cdot \vec{S}_1 + \right. \\
& 2 \hat{n} \cdot \vec{a}_1 \vec{S}_1 \cdot \vec{a}_2 \hat{n} \cdot \vec{S}_1 + 6 \hat{n} \cdot \vec{S}_1 \vec{v}_1 \cdot \vec{a}_2 \hat{n} \cdot \vec{S}_1 + 6 \left( \frac{1}{\vec{S}_1 \cdot \vec{v}_2} \right)^2 + 4 (\hat{n} \cdot \vec{v}_2)^2 \frac{1}{\vec{S}_1 \cdot \vec{S}_1} - 12 \hat{n} \cdot \vec{S}_1 \hat{n} \cdot \vec{v}_2 \vec{S}_1 \cdot \vec{v}_2 -
\end{aligned}$$





$$\begin{aligned}
& 24 \hat{n} \cdot \vec{S}_1 \hat{n} \cdot \vec{v}_2 \vec{S}_1 \cdot \vec{v}_2 (\hat{n} \cdot \vec{v}_1)^2 - 6 \vec{S}_1 \cdot \vec{v}_1 \vec{S}_1 \cdot \vec{v}_2 (\hat{n} \cdot \vec{v}_1)^2 - \frac{15}{2} (\hat{n} \cdot \vec{S}_1)^2 \vec{v}_1 \cdot \vec{v}_2 (\hat{n} \cdot \vec{v}_1)^2 + \\
& \frac{1}{2} \vec{S}_1 \cdot \vec{S}_1 \vec{v}_1 \cdot \vec{v}_2 (\hat{n} \cdot \vec{v}_1)^2 + 6 \hat{n} \cdot \vec{v}_2 (\vec{S}_1 \cdot \vec{v}_1)^2 \hat{n} \cdot \vec{v}_1 + 24 \hat{n} \cdot \vec{S}_1 (\hat{n} \cdot \vec{v}_2)^2 \vec{S}_1 \cdot \vec{v}_1 \hat{n} \cdot \vec{v}_1 + \\
& 4 \hat{n} \cdot \vec{v}_2 \vec{S}_1 \cdot \vec{v}_1 \vec{S}_1 \cdot \vec{v}_2 \hat{n} \cdot \vec{v}_1 + 45 (\hat{n} \cdot \vec{S}_1)^2 \hat{n} \cdot \vec{v}_2 \vec{v}_1 \cdot \vec{v}_1 \hat{n} \cdot \vec{v}_1 - 7 \hat{n} \cdot \vec{v}_2 \vec{S}_1 \cdot \vec{S}_1 \vec{v}_1 \cdot \vec{v}_1 \hat{n} \cdot \vec{v}_1 - \\
& 25 \hat{n} \cdot \vec{S}_1 \vec{S}_1 \cdot \vec{v}_2 \vec{v}_1 \cdot \vec{v}_1 \hat{n} \cdot \vec{v}_1 + 12 (\hat{n} \cdot \vec{S}_1)^2 \hat{n} \cdot \vec{v}_2 \vec{v}_1 \cdot \vec{v}_2 \hat{n} \cdot \vec{v}_1 + 12 \hat{n} \cdot \vec{S}_1 \vec{S}_1 \cdot \vec{v}_1 \vec{v}_1 \cdot \vec{v}_2 \hat{n} \cdot \vec{v}_1 + \\
& 4 \hat{n} \cdot \vec{S}_1 \vec{S}_1 \cdot \vec{v}_2 \vec{v}_1 \cdot \vec{v}_2 \hat{n} \cdot \vec{v}_1 - 4 \hat{n} \cdot \vec{S}_1 \vec{S}_1 \cdot \vec{v}_1 \vec{v}_2 \cdot \vec{v}_2 \hat{n} \cdot \vec{v}_1 - 8 (\hat{n} \cdot \vec{v}_2)^2 (\vec{S}_1 \cdot \vec{v}_1)^2 - \\
& 2 (\hat{n} \cdot \vec{S}_1)^2 (\vec{v}_1 \cdot \vec{v}_2)^2 - 60 (\hat{n} \cdot \vec{S}_1)^2 (\hat{n} \cdot \vec{v}_2)^2 \vec{v}_1 \cdot \vec{v}_1 - 6 (\vec{S}_1 \cdot \vec{v}_2)^2 \vec{v}_1 \cdot \vec{v}_1 + 8 (\hat{n} \cdot \vec{v}_2)^2 \vec{S}_1 \cdot \vec{S}_1 \vec{v}_1 \cdot \vec{v}_1 - \\
& 5 \hat{n} \cdot \vec{S}_1 \hat{n} \cdot \vec{v}_2 \vec{S}_1 \cdot \vec{v}_1 \vec{v}_1 \cdot \vec{v}_1 + 44 \hat{n} \cdot \vec{S}_1 \hat{n} \cdot \vec{v}_2 \vec{S}_1 \cdot \vec{v}_2 \vec{v}_1 \cdot \vec{v}_1 + 4 \vec{S}_1 \cdot \vec{v}_1 \vec{S}_1 \cdot \vec{v}_2 \vec{v}_1 \cdot \vec{v}_1 - \\
& 3 (\vec{S}_1 \cdot \vec{v}_1)^2 \vec{v}_1 \cdot \vec{v}_2 - 20 \hat{n} \cdot \vec{S}_1 \hat{n} \cdot \vec{v}_2 \vec{S}_1 \cdot \vec{v}_1 \vec{v}_1 \cdot \vec{v}_2 + 2 \vec{S}_1 \cdot \vec{v}_1 \vec{S}_1 \cdot \vec{v}_2 \vec{v}_1 \cdot \vec{v}_2 - \frac{5}{2} (\hat{n} \cdot \vec{S}_1)^2 \vec{v}_1 \cdot \vec{v}_1 \vec{v}_1 \cdot \vec{v}_2 + \\
& \frac{1}{2} \vec{S}_1 \cdot \vec{S}_1 \vec{v}_1 \cdot \vec{v}_1 \vec{v}_1 \cdot \vec{v}_2 + 2 (\vec{S}_1 \cdot \vec{v}_1)^2 \vec{v}_2 \cdot \vec{v}_2 + 10 (\hat{n} \cdot \vec{S}_1)^2 \vec{v}_1 \cdot \vec{v}_1 \vec{v}_2 \cdot \vec{v}_2 - 2 \vec{S}_1 \cdot \vec{S}_1 \vec{v}_1 \cdot \vec{v}_1 \vec{v}_2 \cdot \vec{v}_2 \Big) \Big) m_2 C_{ES^2 1} \Big\}
\end{aligned}$$

{DiagS1CES2[2, 2, 30],

,  $\frac{1}{m_1}$

$$\begin{aligned}
& G^2 \left( \frac{8 \hat{n} \cdot \vec{a}_2 \vec{S}_1 \cdot \vec{S}_1 - 8 \hat{n} \cdot \vec{S}_1 \vec{S}_1 \cdot \vec{a}_2 - 4 \hat{n} \cdot \vec{S}_1 \vec{S}_1 \cdot \vec{a}_2 + 8 \hat{n} \cdot \vec{a}_2 \vec{S}_1 \cdot \vec{S}_1 - 4 \hat{n} \cdot \vec{S}_1 \vec{S}_1 \cdot \vec{a}_2}{r} + \frac{1}{r^2} \right. \\
& \left( -8 \vec{v}_2 \cdot \vec{v}_2 (\hat{n} \cdot \vec{S}_1)^2 - 8 \hat{n} \cdot \vec{v}_2 \vec{S}_1 \cdot \vec{v}_2 \hat{n} \cdot \vec{S}_1 + 8 \hat{n} \cdot \vec{v}_1 \vec{S}_1 \cdot \vec{a}_2 \hat{n} \cdot \vec{S}_1 - 4 \hat{n} \cdot \vec{a}_2 \vec{S}_1 \cdot \vec{v}_2 \hat{n} \cdot \vec{S}_1 + 16 \hat{n} \cdot \vec{S}_1 \vec{v}_1 \cdot \vec{a}_2 \hat{n} \cdot \vec{S}_1 + \right. \\
& 8 \hat{n} \cdot \vec{S}_1 \vec{v}_2 \cdot \vec{a}_2 \hat{n} \cdot \vec{S}_1 + 4 (\vec{S}_1 \cdot \vec{v}_2)^2 + 8 (\hat{n} \cdot \vec{v}_2)^2 \vec{S}_1 \cdot \vec{S}_1 + 8 \hat{n} \cdot \vec{S}_1 \hat{n} \cdot \vec{v}_1 \vec{S}_1 \cdot \vec{a}_2 - 4 \hat{n} \cdot \vec{a}_2 \hat{n} \cdot \vec{S}_1 \vec{S}_1 \cdot \vec{v}_2 - \\
& 4 \hat{n} \cdot \vec{S}_1 \hat{n} \cdot \vec{v}_2 \vec{S}_1 \cdot \vec{v}_2 + 8 (\hat{n} \cdot \vec{S}_1)^2 \vec{a}_1 \cdot \vec{a}_2 - 16 \hat{n} \cdot \vec{a}_2 \hat{n} \cdot \vec{v}_1 \vec{S}_1 \cdot \vec{S}_1 + 8 \hat{n} \cdot \vec{a}_2 \hat{n} \cdot \vec{v}_2 \vec{S}_1 \cdot \vec{S}_1 + 8 (\hat{n} \cdot \vec{v}_2)^2 \vec{S}_1 \cdot \vec{S}_1 - \\
& 4 \vec{S}_1 \cdot \vec{v}_1 \vec{S}_1 \cdot \vec{a}_2 + 2 \vec{S}_1 \cdot \vec{v}_2 \vec{S}_1 \cdot \vec{a}_2 - 4 \vec{S}_1 \cdot \vec{a}_2 \vec{S}_1 \cdot \vec{v}_1 - 4 \hat{n} \cdot \vec{S}_1 \hat{n} \cdot \vec{v}_2 \vec{S}_1 \cdot \vec{v}_2 + 2 \vec{S}_1 \cdot \vec{a}_2 \vec{S}_1 \cdot \vec{v}_2 + 4 \vec{S}_1 \cdot \vec{v}_2 \vec{S}_1 \cdot \vec{v}_2 + \\
& 8 \vec{S}_1 \cdot \vec{S}_1 \vec{v}_1 \cdot \vec{a}_2 - 4 \vec{S}_1 \cdot \vec{S}_1 \vec{v}_2 \cdot \vec{a}_2 - 8 \hat{n} \cdot \vec{S}_1 \hat{n} \cdot \vec{S}_1 \vec{v}_2 \cdot \vec{v}_2 - 4 \vec{S}_1 \cdot \vec{S}_1 \vec{v}_2 \cdot \vec{v}_2 - 4 \vec{S}_1 \cdot \vec{S}_1 \vec{v}_2 \cdot \vec{v}_2 \Big) + \frac{1}{r^3} \\
& \left( 8 \vec{S}_1 \cdot \vec{S}_1 (\hat{n} \cdot \vec{v}_2)^3 - 4 \hat{n} \cdot \vec{S}_1 \vec{S}_1 \cdot \vec{v}_2 (\hat{n} \cdot \vec{v}_2)^2 - 32 \hat{n} \cdot \vec{v}_1 \vec{S}_1 \cdot \vec{S}_1 (\hat{n} \cdot \vec{v}_2)^2 - 4 \hat{n} \cdot \vec{S}_1 \vec{S}_1 \cdot \vec{v}_2 (\hat{n} \cdot \vec{v}_2)^2 + \right. \\
& 16 \hat{n} \cdot \vec{S}_1 \hat{n} \cdot \vec{v}_1 \vec{S}_1 \cdot \vec{v}_2 \hat{n} \cdot \vec{v}_2 + 16 (\hat{n} \cdot \vec{S}_1)^2 \vec{a}_1 \cdot \vec{v}_2 \hat{n} \cdot \vec{v}_2 - 4 \vec{S}_1 \cdot \vec{v}_2 \vec{S}_1 \cdot \vec{v}_1 \hat{n} \cdot \vec{v}_2 + 16 \hat{n} \cdot \vec{S}_1 \hat{n} \cdot \vec{v}_1 \vec{S}_1 \cdot \vec{v}_2 \hat{n} \cdot \vec{v}_2 - \\
& 4 \vec{S}_1 \cdot \vec{v}_1 \vec{S}_1 \cdot \vec{v}_2 \hat{n} \cdot \vec{v}_2 + 4 \vec{S}_1 \cdot \vec{v}_2 \vec{S}_1 \cdot \vec{v}_2 \hat{n} \cdot \vec{v}_2 + 32 \hat{n} \cdot \vec{S}_1 \hat{n} \cdot \vec{S}_1 \vec{v}_1 \cdot \vec{v}_2 \hat{n} \cdot \vec{v}_2 + 16 \vec{S}_1 \cdot \vec{S}_1 \vec{v}_1 \cdot \vec{v}_2 \hat{n} \cdot \vec{v}_2 - \\
& 16 \hat{n} \cdot \vec{S}_1 \hat{n} \cdot \vec{S}_1 \vec{v}_2 \cdot \vec{v}_2 \hat{n} \cdot \vec{v}_2 - 4 \vec{S}_1 \cdot \vec{S}_1 \vec{v}_2 \cdot \vec{v}_2 \hat{n} \cdot \vec{v}_2 - 8 \hat{n} \cdot \vec{v}_1 \vec{S}_1 \cdot \vec{v}_2 \vec{S}_1 \cdot \vec{v}_2 - 8 \hat{n} \cdot \vec{S}_1 \vec{a}_1 \cdot \vec{v}_2 \vec{S}_1 \cdot \vec{v}_2 - \\
& 32 (\hat{n} \cdot \vec{S}_1)^2 \hat{n} \cdot \vec{v}_1 \vec{v}_1 \cdot \vec{a}_2 + 16 \hat{n} \cdot \vec{S}_1 \vec{S}_1 \cdot \vec{v}_1 \vec{v}_1 \cdot \vec{a}_2 + 16 \hat{n} \cdot \vec{a}_2 (\hat{n} \cdot \vec{S}_1)^2 \vec{v}_1 \cdot \vec{v}_2 - 12 \hat{n} \cdot \vec{S}_1 \vec{S}_1 \cdot \vec{v}_2 \vec{v}_1 \cdot \vec{v}_2 - \\
& 8 \hat{n} \cdot \vec{S}_1 \vec{S}_1 \cdot \vec{a}_2 \vec{v}_1 \cdot \vec{v}_2 - 12 \hat{n} \cdot \vec{S}_1 \vec{S}_1 \cdot \vec{v}_2 \vec{v}_1 \cdot \vec{v}_2 - 16 (\hat{n} \cdot \vec{S}_1)^2 \hat{n} \cdot \vec{v}_1 \vec{v}_2 \cdot \vec{a}_2 + 8 \hat{n} \cdot \vec{S}_1 \vec{S}_1 \cdot \vec{v}_1 \vec{v}_2 \cdot \vec{a}_2 + \\
& 16 \hat{n} \cdot \vec{a}_1 (\hat{n} \cdot \vec{S}_1)^2 \vec{v}_2 \cdot \vec{v}_2 + 64 \hat{n} \cdot \vec{S}_1 \hat{n} \cdot \vec{S}_1 \hat{n} \cdot \vec{v}_1 \vec{v}_2 \cdot \vec{v}_2 - 16 \hat{n} \cdot \vec{S}_1 \vec{S}_1 \cdot \vec{v}_1 \vec{v}_2 \cdot \vec{v}_2 + 4 \hat{n} \cdot \vec{S}_1 \vec{S}_1 \cdot \vec{v}_2 \vec{v}_2 \cdot \vec{v}_2 + \\
& 8 \hat{n} \cdot \vec{v}_1 \vec{S}_1 \cdot \vec{S}_1 \vec{v}_2 \cdot \vec{v}_2 - 8 \hat{n} \cdot \vec{S}_1 \vec{S}_1 \cdot \vec{a}_1 \vec{v}_2 \cdot \vec{v}_2 - 16 \hat{n} \cdot \vec{S}_1 \vec{S}_1 \cdot \vec{v}_1 \vec{v}_2 \cdot \vec{v}_2 + 4 \hat{n} \cdot \vec{S}_1 \vec{S}_1 \cdot \vec{v}_2 \vec{v}_2 \cdot \vec{v}_2 \Big) + \frac{1}{r^4} \\
& \left( 16 (\vec{v}_1 \cdot \vec{v}_2)^2 (\hat{n} \cdot \vec{S}_1)^2 + 24 (\hat{n} \cdot \vec{v}_2)^2 \vec{v}_1 \cdot \vec{v}_2 (\hat{n} \cdot \vec{S}_1)^2 - 96 \hat{n} \cdot \vec{v}_1 \hat{n} \cdot \vec{v}_2 \vec{v}_1 \cdot \vec{v}_2 (\hat{n} \cdot \vec{S}_1)^2 - 96 (\hat{n} \cdot \vec{v}_1)^2 \right. \\
& \vec{v}_2 \cdot \vec{v}_2 (\hat{n} \cdot \vec{S}_1)^2 + 48 \hat{n} \cdot \vec{v}_1 \hat{n} \cdot \vec{v}_2 \vec{v}_2 \cdot \vec{v}_2 (\hat{n} \cdot \vec{S}_1)^2 + 16 \vec{v}_1 \cdot \vec{v}_1 \vec{v}_2 \cdot \vec{v}_2 (\hat{n} \cdot \vec{S}_1)^2 - 8 \vec{v}_1 \cdot \vec{v}_2 \vec{v}_2 \cdot \vec{v}_2 (\hat{n} \cdot \vec{S}_1)^2 + \\
& 32 \hat{n} \cdot \vec{v}_2 \vec{S}_1 \cdot \vec{v}_1 \vec{v}_1 \cdot \vec{v}_2 \hat{n} \cdot \vec{S}_1 + 32 \hat{n} \cdot \vec{v}_1 \vec{S}_1 \cdot \vec{v}_2 \vec{v}_1 \cdot \vec{v}_2 \hat{n} \cdot \vec{S}_1 - 16 \hat{n} \cdot \vec{v}_2 \vec{S}_1 \cdot \vec{v}_2 \vec{v}_1 \cdot \vec{v}_2 \hat{n} \cdot \vec{S}_1 + \\
& 64 \hat{n} \cdot \vec{v}_1 \vec{S}_1 \cdot \vec{v}_1 \vec{v}_2 \cdot \vec{v}_2 \hat{n} \cdot \vec{S}_1 - 16 \hat{n} \cdot \vec{v}_2 \vec{S}_1 \cdot \vec{v}_1 \vec{v}_2 \cdot \vec{v}_2 \hat{n} \cdot \vec{S}_1 - 16 \hat{n} \cdot \vec{v}_1 \vec{S}_1 \cdot \vec{v}_2 \vec{v}_2 \cdot \vec{v}_2 \hat{n} \cdot \vec{S}_1 + 2 (\vec{S}_1 \cdot \vec{v}_2)^2 \vec{v}_1 \cdot \vec{v}_2 -
\end{aligned}$$

$$\left. 8 \vec{S}_1 \cdot \vec{v}_1 \vec{S}_1 \cdot \vec{v}_2 \vec{v}_1 \cdot \vec{v}_2 - 8 \left( \vec{S}_1 \cdot \vec{v}_1 \right)^2 \vec{v}_2 \cdot \vec{v}_2 + 4 \vec{S}_1 \cdot \vec{v}_1 \vec{S}_1 \cdot \vec{v}_2 \vec{v}_2 \cdot \vec{v}_2 - 2 \vec{S}_1 \cdot \vec{S}_1 \vec{v}_1 \cdot \vec{v}_2 \vec{v}_2 \cdot \vec{v}_2 \right) m_2^2 C_{ES^2_1} \}$$

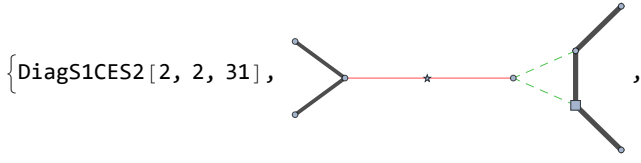

$$\begin{aligned} G^2 \left( \frac{1}{r^2} \left( -4 \hat{n} \cdot \vec{v}_1 \hat{n} \cdot \vec{v}_2 \vec{S}_1 \cdot \vec{S}_1 + 2 \vec{v}_1 \cdot \vec{v}_2 \vec{S}_1 \cdot \vec{S}_1 + 6 \hat{n} \cdot \vec{S}_1 \hat{n} \cdot \vec{v}_2 \vec{S}_1 \cdot \vec{a}_1 + 12 \hat{n} \cdot \vec{S}_1 \hat{n} \cdot \vec{v}_2 \vec{S}_1 \cdot \vec{v}_1 - 6 \vec{S}_1 \cdot \vec{v}_1 \vec{S}_1 \cdot \vec{v}_2 + \right. \right. \\ \left. \left. 6 \hat{n} \cdot \vec{S}_1 \hat{n} \cdot \vec{v}_2 \vec{S}_1 \cdot \vec{v}_1 - 4 \hat{n} \cdot \vec{a}_1 \hat{n} \cdot \vec{v}_2 \vec{S}_1 \cdot \vec{S}_1 + 2 \vec{a}_1 \cdot \vec{v}_2 \vec{S}_1 \cdot \vec{S}_1 - 4 \hat{n} \cdot \vec{v}_1 \hat{n} \cdot \vec{v}_2 \vec{S}_1 \cdot \vec{S}_1 + 6 \hat{n} \cdot \vec{S}_1 \hat{n} \cdot \vec{v}_2 \vec{S}_1 \cdot \vec{a}_1 - \right. \right. \\ \left. \left. 3 \vec{S}_1 \cdot \vec{v}_2 \vec{S}_1 \cdot \vec{a}_1 + 6 \hat{n} \cdot \vec{S}_1 \hat{n} \cdot \vec{v}_2 \vec{S}_1 \cdot \vec{v}_1 - 3 \vec{S}_1 \cdot \vec{v}_2 \vec{S}_1 \cdot \vec{v}_1 - 3 \vec{S}_1 \cdot \vec{a}_1 \vec{S}_1 \cdot \vec{v}_2 - 3 \vec{S}_1 \cdot \vec{v}_1 \vec{S}_1 \cdot \vec{v}_2 + 2 \vec{S}_1 \cdot \vec{S}_1 \vec{v}_1 \cdot \vec{v}_2 \right) + \right. \\ \left. \frac{1}{r^3} \left( -24 \hat{n} \cdot \vec{v}_2 \vec{v}_1 \cdot \vec{a}_1 \left( \hat{n} \cdot \vec{S}_1 \right)^2 - 24 \hat{n} \cdot \vec{v}_1 \hat{n} \cdot \vec{v}_2 \vec{S}_1 \cdot \vec{v}_1 \hat{n} \cdot \vec{S}_1 + 12 \vec{S}_1 \cdot \vec{v}_2 \vec{v}_1 \cdot \vec{a}_1 \hat{n} \cdot \vec{S}_1 - \right. \right. \\ \left. \left. 24 \hat{n} \cdot \vec{S}_1 \hat{n} \cdot \vec{v}_2 \vec{v}_1 \cdot \vec{v}_1 \hat{n} \cdot \vec{S}_1 + 6 \vec{S}_1 \cdot \vec{v}_2 \vec{v}_1 \cdot \vec{v}_1 \hat{n} \cdot \vec{S}_1 + 6 \vec{S}_1 \cdot \vec{v}_1 \vec{v}_1 \cdot \vec{v}_2 \hat{n} \cdot \vec{S}_1 + 16 \left( \hat{n} \cdot \vec{v}_1 \right)^2 \hat{n} \cdot \vec{v}_2 \vec{S}_1 \cdot \vec{S}_1 - \right. \right. \\ \left. \left. 24 \hat{n} \cdot \vec{S}_1 \hat{n} \cdot \vec{v}_1 \hat{n} \cdot \vec{v}_2 \vec{S}_1 \cdot \vec{v}_1 + 12 \hat{n} \cdot \vec{v}_2 \vec{S}_1 \cdot \vec{v}_1 \vec{S}_1 \cdot \vec{v}_1 + 6 \hat{n} \cdot \vec{v}_1 \vec{S}_1 \cdot \vec{v}_2 \vec{S}_1 \cdot \vec{v}_1 + 6 \hat{n} \cdot \vec{v}_1 \vec{S}_1 \cdot \vec{v}_1 \vec{S}_1 \cdot \vec{v}_2 + \right. \right. \\ \left. \left. 4 \hat{n} \cdot \vec{v}_2 \vec{S}_1 \cdot \vec{S}_1 \vec{v}_1 \cdot \vec{a}_1 + 6 \hat{n} \cdot \vec{S}_1 \vec{S}_1 \cdot \vec{v}_2 \vec{v}_1 \cdot \vec{v}_1 - 8 \hat{n} \cdot \vec{v}_1 \vec{S}_1 \cdot \vec{S}_1 \vec{v}_1 \cdot \vec{v}_2 + 6 \hat{n} \cdot \vec{S}_1 \vec{S}_1 \cdot \vec{v}_1 \vec{v}_1 \cdot \vec{v}_2 \right) + \frac{1}{r^4} \right. \\ \left. \left( 72 \hat{n} \cdot \vec{v}_1 \hat{n} \cdot \vec{v}_2 \vec{v}_1 \cdot \vec{v}_1 \left( \hat{n} \cdot \vec{S}_1 \right)^2 - 12 \vec{v}_1 \cdot \vec{v}_1 \vec{v}_1 \cdot \vec{v}_2 \left( \hat{n} \cdot \vec{S}_1 \right)^2 - 24 \hat{n} \cdot \vec{v}_2 \vec{S}_1 \cdot \vec{v}_1 \vec{v}_1 \cdot \vec{v}_1 \hat{n} \cdot \vec{S}_1 - 24 \hat{n} \cdot \vec{v}_1 \right. \right. \\ \left. \left. \vec{S}_1 \cdot \vec{v}_2 \vec{v}_1 \cdot \vec{v}_1 \hat{n} \cdot \vec{S}_1 - 8 \hat{n} \cdot \vec{v}_1 \hat{n} \cdot \vec{v}_2 \vec{S}_1 \cdot \vec{S}_1 \vec{v}_1 \cdot \vec{v}_1 + 6 \vec{S}_1 \cdot \vec{v}_1 \vec{S}_1 \cdot \vec{v}_2 \vec{v}_1 \cdot \vec{v}_1 + 2 \vec{S}_1 \cdot \vec{S}_1 \vec{v}_1 \cdot \vec{v}_1 \vec{v}_1 \cdot \vec{v}_2 \right) \right) m_2 C_{ES^2_1} \} \end{aligned}$$

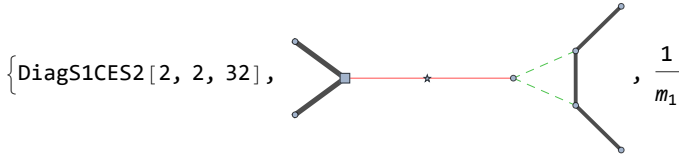

$$\begin{aligned} G^2 m_2^2 C_{ES^2_1} \left( \frac{1}{r^3} \left( 32 \vec{v}_2 \cdot \vec{a}_2 \left( \hat{n} \cdot \vec{S}_1 \right)^2 \hat{n} \cdot \vec{v}_1 - 16 \vec{v}_2 \cdot \vec{a}_2 \hat{n} \cdot \vec{S}_1 \vec{S}_1 \cdot \vec{v}_1 - 32 \vec{v}_2 \cdot \vec{v}_2 \hat{n} \cdot \vec{S}_1 \hat{n} \cdot \vec{S}_1 \hat{n} \cdot \vec{v}_2 + 8 \vec{v}_2 \cdot \vec{v}_2 \hat{n} \cdot \vec{S}_1 \vec{S}_1 \cdot \vec{v}_2 + \right. \right. \\ \left. \left. 8 \vec{v}_2 \cdot \vec{v}_2 \hat{n} \cdot \vec{S}_1 \vec{S}_1 \cdot \vec{v}_2 \right) - \frac{16 \vec{v}_2 \cdot \vec{a}_2 \hat{n} \cdot \vec{S}_1 \hat{n} \cdot \vec{S}_1}{r^2} + \frac{1}{r^4} \left( 96 \vec{v}_2 \cdot \vec{v}_2 \left( \hat{n} \cdot \vec{S}_1 \right)^2 \hat{n} \cdot \vec{v}_1 \hat{n} \cdot \vec{v}_2 - 16 \vec{v}_1 \cdot \vec{v}_2 \vec{v}_2 \cdot \vec{v}_2 \left( \hat{n} \cdot \vec{S}_1 \right)^2 - \right. \right. \\ \left. \left. 32 \vec{v}_2 \cdot \vec{v}_2 \hat{n} \cdot \vec{S}_1 \hat{n} \cdot \vec{v}_2 \vec{S}_1 \cdot \vec{v}_1 - 32 \vec{v}_2 \cdot \vec{v}_2 \hat{n} \cdot \vec{S}_1 \hat{n} \cdot \vec{v}_1 \vec{S}_1 \cdot \vec{v}_2 + 8 \vec{v}_2 \cdot \vec{v}_2 \vec{S}_1 \cdot \vec{v}_1 \vec{S}_1 \cdot \vec{v}_2 \right) \right) \} \end{aligned}$$

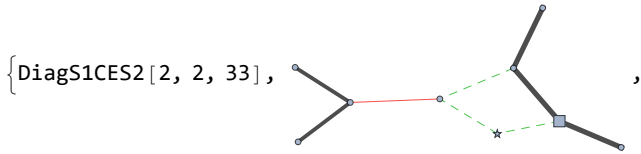

$$\begin{aligned} G^2 \left( \frac{-4 \hat{n} \cdot \vec{a}_1 \vec{S}_1 \cdot \vec{S}_1 - 4 \hat{n} \cdot \vec{S}_1 \vec{S}_1 \cdot \vec{a}_1 - 2 \hat{n} \cdot \vec{S}_1 \vec{S}_1 \cdot \vec{a}_1 - 4 \hat{n} \cdot \vec{a}_1 \vec{S}_1 \cdot \vec{S}_1 - 2 \hat{n} \cdot \vec{S}_1 \vec{S}_1 \cdot \vec{a}_1}{r} + \frac{1}{r^2} \right. \\ \left. \left( -2 \vec{v}_1 \cdot \vec{v}_1 \left( \hat{n} \cdot \vec{S}_1 \right)^2 + 6 \hat{n} \cdot \vec{v}_1 \vec{S}_1 \cdot \vec{v}_1 \hat{n} \cdot \vec{S}_1 - 8 \hat{n} \cdot \vec{v}_2 \vec{S}_1 \cdot \vec{v}_1 \hat{n} \cdot \vec{S}_1 + 4 \hat{n} \cdot \vec{v}_1 \vec{S}_1 \cdot \vec{a}_1 \hat{n} \cdot \vec{S}_1 - 3 \hat{n} \cdot \vec{a}_1 \vec{S}_1 \cdot \vec{v}_1 \hat{n} \cdot \vec{S}_1 + \right. \right. \end{aligned}$$

$$\begin{aligned}
& 4 \hat{n} \cdot \vec{S}_1 \vec{v}_1 \cdot \vec{a}_1 \hat{n} \cdot \vec{S}_1 - 6 \left( \vec{S}_1 \cdot \vec{v}_1 \right)^2 + 6 \left( \hat{n} \cdot \vec{v}_1 \right)^2 \vec{S}_1 \cdot \vec{S}_1 - 8 \hat{n} \cdot \vec{v}_1 \hat{n} \cdot \vec{v}_2 \vec{S}_1 \cdot \vec{S}_1 + 4 \hat{n} \cdot \vec{S}_1 \hat{n} \cdot \vec{v}_1 \vec{S}_1 \cdot \vec{a}_1 - \\
& 3 \hat{n} \cdot \vec{a}_1 \hat{n} \cdot \vec{S}_1 \vec{S}_1 \cdot \vec{v}_1 + 4 \vec{S}_1 \cdot \vec{v}_1 \vec{S}_1 \cdot \vec{v}_2 + 3 \hat{n} \cdot \vec{S}_1 \hat{n} \cdot \vec{v}_1 \vec{S}_1 \cdot \vec{v}_1 - 4 \hat{n} \cdot \vec{S}_1 \hat{n} \cdot \vec{v}_2 \vec{S}_1 \cdot \vec{v}_1 + \left( \hat{n} \cdot \vec{S}_1 \right)^2 \vec{a}_1 \cdot \vec{a}_1 + \\
& 2 \hat{n} \cdot \vec{a}_1 \hat{n} \cdot \vec{v}_1 \vec{S}_1 \cdot \vec{S}_1 + 6 \left( \hat{n} \cdot \vec{v}_1 \right)^2 \vec{S}_1 \cdot \vec{S}_1 - 8 \hat{n} \cdot \vec{v}_1 \hat{n} \cdot \vec{v}_2 \vec{S}_1 \cdot \vec{S}_1 + \vec{S}_1 \cdot \vec{v}_1 \vec{S}_1 \cdot \vec{a}_1 - 3 \vec{a}_1 \cdot \vec{a}_1 \vec{S}_1 \cdot \vec{S}_1 + \\
& 3 \hat{n} \cdot \vec{S}_1 \hat{n} \cdot \vec{v}_1 \vec{S}_1 \cdot \vec{v}_1 - 4 \hat{n} \cdot \vec{S}_1 \hat{n} \cdot \vec{v}_2 \vec{S}_1 \cdot \vec{v}_1 + \vec{S}_1 \cdot \vec{a}_1 \vec{S}_1 \cdot \vec{v}_1 - 6 \vec{S}_1 \cdot \vec{v}_1 \vec{S}_1 \cdot \vec{v}_1 + 2 \vec{S}_1 \cdot \vec{v}_2 \vec{S}_1 \cdot \vec{v}_1 + \\
& 2 \vec{S}_1 \cdot \vec{v}_1 \vec{S}_1 \cdot \vec{v}_2 - 10 \vec{S}_1 \cdot \vec{S}_1 \vec{v}_1 \cdot \vec{a}_1 - 2 \hat{n} \cdot \vec{S}_1 \hat{n} \cdot \vec{S}_1 \vec{v}_1 \cdot \vec{v}_1 + 4 \vec{S}_1 \cdot \vec{S}_1 \vec{v}_1 \cdot \vec{v}_2 + 4 \vec{S}_1 \cdot \vec{S}_1 \vec{v}_1 \cdot \vec{v}_2 \Big) + \frac{1}{r^3} \\
& \left( -4 \vec{S}_1 \cdot \vec{S}_1 \left( \hat{n} \cdot \vec{v}_1 \right)^3 - 2 \hat{n} \cdot \vec{S}_1 \vec{S}_1 \cdot \vec{v}_1 \left( \hat{n} \cdot \vec{v}_1 \right)^2 + 8 \hat{n} \cdot \vec{v}_2 \vec{S}_1 \cdot \vec{S}_1 \left( \hat{n} \cdot \vec{v}_1 \right)^2 - 2 \hat{n} \cdot \vec{S}_1 \vec{S}_1 \cdot \vec{v}_1 \left( \hat{n} \cdot \vec{v}_1 \right)^2 + \right. \\
& 4 \hat{n} \cdot \vec{S}_1 \hat{n} \cdot \vec{v}_2 \vec{S}_1 \cdot \vec{v}_1 \hat{n} \cdot \vec{v}_1 - 8 \hat{n} \cdot \vec{S}_1 \hat{n} \cdot \vec{v}_2 \vec{S}_1 \cdot \vec{a}_1 \hat{n} \cdot \vec{v}_1 + 4 \hat{n} \cdot \vec{S}_1 \hat{n} \cdot \vec{v}_2 \vec{S}_1 \cdot \vec{v}_1 \hat{n} \cdot \vec{v}_1 - 2 \vec{S}_1 \cdot \vec{v}_1 \vec{S}_1 \cdot \vec{v}_1 \hat{n} \cdot \vec{v}_1 - \\
& \vec{S}_1 \cdot \vec{v}_2 \vec{S}_1 \cdot \vec{v}_1 \hat{n} \cdot \vec{v}_1 - 2 \vec{S}_1 \cdot \vec{a}_1 \vec{S}_1 \cdot \vec{v}_1 \hat{n} \cdot \vec{v}_1 - \vec{S}_1 \cdot \vec{v}_1 \vec{S}_1 \cdot \vec{v}_2 \hat{n} \cdot \vec{v}_1 + 2 \vec{S}_1 \cdot \vec{a}_1 \vec{S}_1 \cdot \vec{v}_2 \hat{n} \cdot \vec{v}_1 - \\
& 8 \left( \hat{n} \cdot \vec{S}_1 \right)^2 \vec{v}_1 \cdot \vec{a}_1 \hat{n} \cdot \vec{v}_1 + 10 \vec{S}_1 \cdot \vec{S}_1 \vec{v}_1 \cdot \vec{a}_1 \hat{n} \cdot \vec{v}_1 + 8 \vec{S}_1 \cdot \vec{S}_1 \vec{v}_1 \cdot \vec{v}_1 \hat{n} \cdot \vec{v}_1 - 4 \vec{S}_1 \cdot \vec{S}_1 \vec{v}_1 \cdot \vec{v}_2 \hat{n} \cdot \vec{v}_1 + \\
& 2 \hat{n} \cdot \vec{a}_1 \left( \vec{S}_1 \cdot \vec{v}_1 \right)^2 + 8 \hat{n} \cdot \vec{a}_1 \hat{n} \cdot \vec{S}_1 \hat{n} \cdot \vec{v}_2 \vec{S}_1 \cdot \vec{v}_1 + 4 \hat{n} \cdot \vec{v}_2 \vec{S}_1 \cdot \vec{v}_1 \vec{S}_1 \cdot \vec{v}_1 - 2 \hat{n} \cdot \vec{S}_1 \vec{a}_1 \cdot \vec{v}_2 \vec{S}_1 \cdot \vec{v}_1 - \\
& 2 \hat{n} \cdot \vec{a}_1 \vec{S}_1 \cdot \vec{v}_1 \vec{S}_1 \cdot \vec{v}_2 + 4 \left( \hat{n} \cdot \vec{S}_1 \right)^2 \hat{n} \cdot \vec{v}_2 \vec{v}_1 \cdot \vec{a}_1 - 6 \hat{n} \cdot \vec{v}_2 \vec{S}_1 \cdot \vec{S}_1 \vec{v}_1 \cdot \vec{a}_1 + 4 \hat{n} \cdot \vec{S}_1 \vec{S}_1 \cdot \vec{v}_1 \vec{v}_1 \cdot \vec{a}_1 - \\
& 2 \hat{n} \cdot \vec{S}_1 \vec{S}_1 \cdot \vec{v}_2 \vec{v}_1 \cdot \vec{a}_1 + 4 \hat{n} \cdot \vec{a}_1 \left( \hat{n} \cdot \vec{S}_1 \right)^2 \vec{v}_1 \cdot \vec{v}_1 + 16 \hat{n} \cdot \vec{S}_1 \hat{n} \cdot \vec{S}_1 \hat{n} \cdot \vec{v}_2 \vec{v}_1 \cdot \vec{v}_1 + 5 \hat{n} \cdot \vec{S}_1 \vec{S}_1 \cdot \vec{v}_1 \vec{v}_1 \cdot \vec{v}_1 - \\
& 4 \hat{n} \cdot \vec{S}_1 \vec{S}_1 \cdot \vec{v}_2 \vec{v}_1 \cdot \vec{v}_1 - 20 \hat{n} \cdot \vec{v}_2 \vec{S}_1 \cdot \vec{S}_1 \vec{v}_1 \cdot \vec{v}_1 - 2 \hat{n} \cdot \vec{S}_1 \vec{S}_1 \cdot \vec{a}_1 \vec{v}_1 \cdot \vec{v}_1 - 4 \hat{n} \cdot \vec{a}_1 \vec{S}_1 \cdot \vec{S}_1 \vec{v}_1 \cdot \vec{v}_1 + \\
& 5 \hat{n} \cdot \vec{S}_1 \vec{S}_1 \cdot \vec{v}_1 \vec{v}_1 \cdot \vec{v}_1 - 4 \hat{n} \cdot \vec{S}_1 \vec{S}_1 \cdot \vec{v}_2 \vec{v}_1 \cdot \vec{v}_1 - \hat{n} \cdot \vec{S}_1 \vec{S}_1 \cdot \vec{v}_1 \vec{v}_1 \cdot \vec{v}_2 + 2 \hat{n} \cdot \vec{S}_1 \vec{S}_1 \cdot \vec{a}_1 \vec{v}_1 \cdot \vec{v}_2 - \hat{n} \cdot \vec{S}_1 \vec{S}_1 \cdot \vec{v}_1 \vec{v}_1 \cdot \vec{v}_2 \Big) + \\
& \frac{1}{r^4} \left( -\frac{5}{2} \left( \vec{v}_1 \cdot \vec{v}_1 \right)^2 \left( \hat{n} \cdot \vec{S}_1 \right)^2 + \frac{3}{2} \left( \hat{n} \cdot \vec{v}_1 \right)^2 \vec{v}_1 \cdot \vec{v}_1 \left( \hat{n} \cdot \vec{S}_1 \right)^2 - 24 \hat{n} \cdot \vec{v}_1 \hat{n} \cdot \vec{v}_2 \vec{v}_1 \cdot \vec{v}_1 \left( \hat{n} \cdot \vec{S}_1 \right)^2 + \right. \\
& 4 \vec{v}_1 \cdot \vec{v}_1 \vec{v}_1 \cdot \vec{v}_2 \left( \hat{n} \cdot \vec{S}_1 \right)^2 - 2 \hat{n} \cdot \vec{v}_1 \vec{S}_1 \cdot \vec{v}_1 \vec{v}_1 \cdot \vec{v}_1 \hat{n} \cdot \vec{S}_1 + 8 \hat{n} \cdot \vec{v}_1 \vec{S}_1 \cdot \vec{v}_2 \vec{v}_1 \cdot \vec{v}_1 \hat{n} \cdot \vec{S}_1 + \frac{1}{2} \vec{S}_1 \cdot \vec{S}_1 \left( \vec{v}_1 \cdot \vec{v}_1 \right)^2 + \\
& \left. \left( \vec{S}_1 \cdot \vec{v}_1 \right)^2 \vec{v}_1 \cdot \vec{v}_1 - \frac{5}{2} \left( \hat{n} \cdot \vec{v}_1 \right)^2 \vec{S}_1 \cdot \vec{S}_1 \vec{v}_1 \cdot \vec{v}_1 + 16 \hat{n} \cdot \vec{v}_1 \hat{n} \cdot \vec{v}_2 \vec{S}_1 \cdot \vec{S}_1 \vec{v}_1 \cdot \vec{v}_1 - 4 \vec{S}_1 \cdot \vec{S}_1 \vec{v}_1 \cdot \vec{v}_1 \vec{v}_1 \cdot \vec{v}_2 \right) \Bigg\} m_2 C_{ES^2_1}
\end{aligned}$$

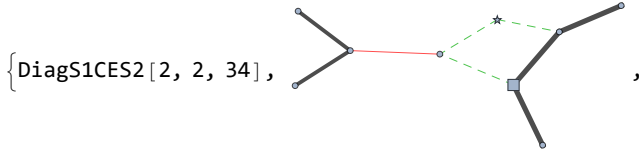

$$\begin{aligned}
& G^2 \left( \frac{4 \hat{n} \cdot \vec{a}_1 \vec{S}_1 \cdot \vec{S}_1 - 12 \hat{n} \cdot \vec{S}_1 \vec{S}_1 \cdot \vec{a}_1 - 6 \hat{n} \cdot \vec{S}_1 \vec{S}_1 \cdot \vec{a}_1 + 4 \hat{n} \cdot \vec{a}_1 \vec{S}_1 \cdot \vec{S}_1 - 6 \hat{n} \cdot \vec{S}_1 \vec{S}_1 \cdot \vec{a}_1}{r} + \frac{1}{r^2} \right. \\
& \left( -6 \vec{v}_1 \cdot \vec{v}_1 \left( \hat{n} \cdot \vec{S}_1 \right)^2 + 6 \hat{n} \cdot \vec{v}_1 \vec{S}_1 \cdot \vec{v}_1 \hat{n} \cdot \vec{S}_1 + 18 \hat{n} \cdot \vec{v}_1 \vec{S}_1 \cdot \vec{a}_1 \hat{n} \cdot \vec{S}_1 - 12 \hat{n} \cdot \vec{v}_2 \vec{S}_1 \cdot \vec{a}_1 \hat{n} \cdot \vec{S}_1 - \right. \\
& 9 \hat{n} \cdot \vec{a}_1 \vec{S}_1 \cdot \vec{v}_1 \hat{n} \cdot \vec{S}_1 + 24 \hat{n} \cdot \vec{S}_1 \vec{v}_1 \cdot \vec{a}_1 \hat{n} \cdot \vec{S}_1 - 6 \left( \vec{S}_1 \cdot \vec{v}_1 \right)^2 - 2 \left( \hat{n} \cdot \vec{v}_1 \right)^2 \vec{S}_1 \cdot \vec{S}_1 + 18 \hat{n} \cdot \vec{S}_1 \hat{n} \cdot \vec{v}_1 \vec{S}_1 \cdot \vec{a}_1 - \\
& 12 \hat{n} \cdot \vec{S}_1 \hat{n} \cdot \vec{v}_2 \vec{S}_1 \cdot \vec{a}_1 - 9 \hat{n} \cdot \vec{a}_1 \hat{n} \cdot \vec{S}_1 \vec{S}_1 \cdot \vec{v}_1 + 3 \hat{n} \cdot \vec{S}_1 \hat{n} \cdot \vec{v}_1 \vec{S}_1 \cdot \vec{v}_1 + 9 \left( \hat{n} \cdot \vec{S}_1 \right)^2 \vec{a}_1 \cdot \vec{a}_1 - \\
& 6 \hat{n} \cdot \vec{a}_1 \hat{n} \cdot \vec{v}_1 \vec{S}_1 \cdot \vec{S}_1 + 8 \hat{n} \cdot \vec{a}_1 \hat{n} \cdot \vec{v}_2 \vec{S}_1 \cdot \vec{S}_1 - 4 \vec{a}_1 \cdot \vec{v}_2 \vec{S}_1 \cdot \vec{S}_1 - 2 \left( \hat{n} \cdot \vec{v}_1 \right)^2 \vec{S}_1 \cdot \vec{S}_1 - 3 \vec{S}_1 \cdot \vec{v}_1 \vec{S}_1 \cdot \vec{a}_1 + \\
& 6 \vec{S}_1 \cdot \vec{v}_2 \vec{S}_1 \cdot \vec{a}_1 - 3 \vec{a}_1 \cdot \vec{a}_1 \vec{S}_1 \cdot \vec{S}_1 + 3 \hat{n} \cdot \vec{S}_1 \hat{n} \cdot \vec{v}_1 \vec{S}_1 \cdot \vec{v}_1 - 3 \vec{S}_1 \cdot \vec{a}_1 \vec{S}_1 \cdot \vec{v}_1 - 6 \vec{S}_1 \cdot \vec{v}_1 \vec{S}_1 \cdot \vec{v}_1 + \\
& \left. \left. 6 \vec{S}_1 \cdot \vec{a}_1 \vec{S}_1 \cdot \vec{v}_2 - 6 \vec{S}_1 \cdot \vec{S}_1 \vec{v}_1 \cdot \vec{a}_1 - 6 \hat{n} \cdot \vec{S}_1 \hat{n} \cdot \vec{S}_1 \vec{v}_1 \cdot \vec{v}_1 + 4 \vec{S}_1 \cdot \vec{S}_1 \vec{v}_1 \cdot \vec{v}_1 + 4 \vec{S}_1 \cdot \vec{S}_1 \vec{v}_1 \cdot \vec{v}_1 \right) + \frac{1}{r^3} \right)
\end{aligned}$$

$$\begin{aligned}
& \left( 4 \vec{S}_1 \cdot \vec{S}_1 (\hat{n} \cdot \vec{v}_1)^3 - 6 \hat{n} \cdot \vec{S}_1 \vec{S}_1 \cdot \vec{v}_1 (\hat{n} \cdot \vec{v}_1)^2 - 8 \hat{n} \cdot \vec{v}_2 \vec{S}_1 \cdot \vec{S}_1 (\hat{n} \cdot \vec{v}_1)^2 - 16 \hat{n} \cdot \vec{S}_1 \vec{S}_1 \cdot \vec{a}_1 (\hat{n} \cdot \vec{v}_1)^2 - \right. \\
& 6 \hat{n} \cdot \vec{S}_1 \vec{S}_1 \cdot \vec{v}_1 (\hat{n} \cdot \vec{v}_1)^2 + 12 \hat{n} \cdot \vec{S}_1 \hat{n} \cdot \vec{v}_2 \vec{S}_1 \cdot \vec{v}_1 \hat{n} \cdot \vec{v}_1 + 24 \hat{n} \cdot \vec{S}_1 \hat{n} \cdot \vec{v}_2 \vec{S}_1 \cdot \vec{a}_1 \hat{n} \cdot \vec{v}_1 + 16 \hat{n} \cdot \vec{a}_1 \hat{n} \cdot \vec{S}_1 \vec{S}_1 \cdot \vec{v}_1 \hat{n} \cdot \vec{v}_1 + \\
& 12 \hat{n} \cdot \vec{S}_1 \hat{n} \cdot \vec{v}_2 \vec{S}_1 \cdot \vec{v}_1 \hat{n} \cdot \vec{v}_1 + 6 \vec{S}_1 \cdot \vec{v}_1 \vec{S}_1 \cdot \vec{v}_1 \hat{n} \cdot \vec{v}_1 - 3 \vec{S}_1 \cdot \vec{v}_2 \vec{S}_1 \cdot \vec{v}_1 \hat{n} \cdot \vec{v}_1 + 2 \vec{S}_1 \cdot \vec{a}_1 \vec{S}_1 \cdot \vec{v}_1 \hat{n} \cdot \vec{v}_1 - \\
& 3 \vec{S}_1 \cdot \vec{v}_1 \vec{S}_1 \cdot \vec{v}_2 \hat{n} \cdot \vec{v}_1 - 6 \vec{S}_1 \cdot \vec{a}_1 \vec{S}_1 \cdot \vec{v}_2 \hat{n} \cdot \vec{v}_1 - 56 (\hat{n} \cdot \vec{S}_1)^2 \vec{v}_1 \cdot \vec{a}_1 \hat{n} \cdot \vec{v}_1 + 10 \vec{S}_1 \cdot \vec{S}_1 \vec{v}_1 \cdot \vec{a}_1 \hat{n} \cdot \vec{v}_1 + \\
& 24 \hat{n} \cdot \vec{S}_1 \hat{n} \cdot \vec{S}_1 \vec{v}_1 \cdot \vec{v}_1 \hat{n} \cdot \vec{v}_1 - 12 \vec{S}_1 \cdot \vec{S}_1 \vec{v}_1 \cdot \vec{v}_1 \hat{n} \cdot \vec{v}_1 + 4 \vec{S}_1 \cdot \vec{S}_1 \vec{v}_1 \cdot \vec{v}_2 \hat{n} \cdot \vec{v}_1 - 2 \hat{n} \cdot \vec{a}_1 (\vec{S}_1 \cdot \vec{v}_1)^2 - \\
& 24 \hat{n} \cdot \vec{a}_1 \hat{n} \cdot \vec{S}_1 \hat{n} \cdot \vec{v}_2 \vec{S}_1 \cdot \vec{v}_1 - 12 \hat{n} \cdot \vec{v}_2 \vec{S}_1 \cdot \vec{v}_1 \vec{S}_1 \cdot \vec{v}_1 + 6 \hat{n} \cdot \vec{S}_1 \vec{a}_1 \cdot \vec{v}_2 \vec{S}_1 \cdot \vec{v}_1 + 6 \hat{n} \cdot \vec{a}_1 \vec{S}_1 \cdot \vec{v}_1 \vec{S}_1 \cdot \vec{v}_2 + \\
& 36 (\hat{n} \cdot \vec{S}_1)^2 \hat{n} \cdot \vec{v}_2 \vec{v}_1 \cdot \vec{a}_1 - 6 \hat{n} \cdot \vec{v}_2 \vec{S}_1 \cdot \vec{S}_1 \vec{v}_1 \cdot \vec{a}_1 + 24 \hat{n} \cdot \vec{S}_1 \vec{S}_1 \cdot \vec{v}_1 \vec{v}_1 \cdot \vec{a}_1 - 18 \hat{n} \cdot \vec{S}_1 \vec{S}_1 \cdot \vec{v}_2 \vec{v}_1 \cdot \vec{a}_1 + \\
& 20 \hat{n} \cdot \vec{a}_1 (\hat{n} \cdot \vec{S}_1)^2 \vec{v}_1 \cdot \vec{v}_1 - 24 \hat{n} \cdot \vec{S}_1 \hat{n} \cdot \vec{S}_1 \hat{n} \cdot \vec{v}_2 \vec{v}_1 \cdot \vec{v}_1 + 3 \hat{n} \cdot \vec{S}_1 \vec{S}_1 \cdot \vec{v}_1 \vec{v}_1 \cdot \vec{v}_1 + 6 \hat{n} \cdot \vec{S}_1 \vec{S}_1 \cdot \vec{v}_2 \vec{v}_1 \cdot \vec{v}_1 + \\
& 8 \hat{n} \cdot \vec{v}_2 \vec{S}_1 \cdot \vec{S}_1 \vec{v}_1 \cdot \vec{v}_1 - 6 \hat{n} \cdot \vec{S}_1 \vec{S}_1 \cdot \vec{a}_1 \vec{v}_1 \cdot \vec{v}_1 - 4 \hat{n} \cdot \vec{a}_1 \vec{S}_1 \cdot \vec{S}_1 \vec{v}_1 \cdot \vec{v}_1 + 3 \hat{n} \cdot \vec{S}_1 \vec{S}_1 \cdot \vec{v}_1 \vec{v}_1 \cdot \vec{v}_1 + \\
& 6 \hat{n} \cdot \vec{S}_1 \vec{S}_1 \cdot \vec{v}_2 \vec{v}_1 \cdot \vec{v}_1 - 3 \hat{n} \cdot \vec{S}_1 \vec{S}_1 \cdot \vec{v}_1 \vec{v}_1 \cdot \vec{v}_2 - 6 \hat{n} \cdot \vec{S}_1 \vec{S}_1 \cdot \vec{a}_1 \vec{v}_1 \cdot \vec{v}_2 - 3 \hat{n} \cdot \vec{S}_1 \vec{S}_1 \cdot \vec{v}_1 \vec{v}_1 \cdot \vec{v}_2 \Big) + \\
& \frac{1}{r^4} \left( -\frac{5}{2} (\vec{v}_1 \cdot \vec{v}_1)^2 (\hat{n} \cdot \vec{S}_1)^2 - \frac{45}{2} (\hat{n} \cdot \vec{v}_1)^2 \vec{v}_1 \cdot \vec{v}_1 (\hat{n} \cdot \vec{S}_1)^2 + 24 \hat{n} \cdot \vec{v}_1 \hat{n} \cdot \vec{v}_2 \vec{v}_1 \cdot \vec{v}_1 (\hat{n} \cdot \vec{S}_1)^2 - \right. \\
& 4 \vec{v}_1 \cdot \vec{v}_1 \vec{v}_1 \cdot \vec{v}_2 (\hat{n} \cdot \vec{S}_1)^2 + 6 \hat{n} \cdot \vec{v}_1 \vec{S}_1 \cdot \vec{v}_1 \vec{v}_1 \cdot \vec{v}_1 \hat{n} \cdot \vec{S}_1 + 8 \hat{n} \cdot \vec{v}_2 \vec{S}_1 \cdot \vec{v}_1 \vec{v}_1 \cdot \vec{v}_1 \hat{n} \cdot \vec{S}_1 - \\
& 8 \hat{n} \cdot \vec{v}_1 \vec{S}_1 \cdot \vec{v}_2 \vec{v}_1 \cdot \vec{v}_1 \hat{n} \cdot \vec{S}_1 + \frac{1}{2} \vec{S}_1 \cdot \vec{S}_1 (\vec{v}_1 \cdot \vec{v}_1)^2 + (\vec{S}_1 \cdot \vec{v}_1)^2 \vec{v}_1 \cdot \vec{v}_1 + \frac{11}{2} (\hat{n} \cdot \vec{v}_1)^2 \vec{S}_1 \cdot \vec{S}_1 \vec{v}_1 \cdot \vec{v}_1 - \\
& \left. 8 \hat{n} \cdot \vec{v}_1 \hat{n} \cdot \vec{v}_2 \vec{S}_1 \cdot \vec{S}_1 \vec{v}_1 \cdot \vec{v}_1 - 2 \vec{S}_1 \cdot \vec{v}_1 \vec{S}_1 \cdot \vec{v}_2 \vec{v}_1 \cdot \vec{v}_1 + 2 \vec{S}_1 \cdot \vec{S}_1 \vec{v}_1 \cdot \vec{v}_1 \vec{v}_1 \cdot \vec{v}_2 \right) \Bigg\} m_2 C_{ES^2_1} \Bigg\}
\end{aligned}$$

{DiagS1CES2[2, 2, 35],

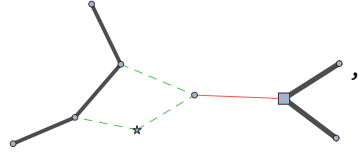

$$\begin{aligned}
& \frac{1}{m_1} G^2 m_2^2 C_{ES^2_1} \left( \frac{1}{r^3} \left( -32 \vec{v}_2 \cdot \vec{a}_2 (\hat{n} \cdot \vec{S}_1)^2 \hat{n} \cdot \vec{v}_1 + 64 \vec{v}_2 \cdot \vec{a}_2 (\hat{n} \cdot \vec{S}_1)^2 \hat{n} \cdot \vec{v}_2 - \right. \right. \\
& 32 \vec{v}_2 \cdot \vec{v}_2 \hat{n} \cdot \vec{a}_2 (\hat{n} \cdot \vec{S}_1)^2 + 16 \vec{v}_2 \cdot \vec{a}_2 \hat{n} \cdot \vec{S}_1 \vec{S}_1 \cdot \vec{v}_1 - 32 \vec{v}_2 \cdot \vec{a}_2 \hat{n} \cdot \vec{S}_1 \vec{S}_1 \cdot \vec{v}_2 + 16 \vec{v}_2 \cdot \vec{v}_2 \vec{S}_1 \cdot \vec{a}_2 \hat{n} \cdot \vec{S}_1 \Big) + \\
& \frac{16 \vec{v}_2 \cdot \vec{a}_2 \hat{n} \cdot \vec{S}_1 \hat{n} \cdot \vec{S}_1 + 8 \vec{a}_2 \cdot \vec{a}_2 (\hat{n} \cdot \vec{S}_1)^2}{r^2} + \frac{1}{r^4} \left( -24 \vec{v}_2 \cdot \vec{v}_2 (\hat{n} \cdot \vec{S}_1)^2 (\hat{n} \cdot \vec{v}_2)^2 + \right. \\
& \left. 16 \vec{v}_2 \cdot \vec{v}_2 \hat{n} \cdot \vec{S}_1 \hat{n} \cdot \vec{v}_2 \vec{S}_1 \cdot \vec{v}_2 - 8 (\vec{v}_2 \cdot \vec{v}_2)^2 (\hat{n} \cdot \vec{S}_1)^2 + 6 \vec{S}_1 \cdot \vec{S}_1 (\vec{v}_2 \cdot \vec{v}_2)^2 - 2 \vec{v}_2 \cdot \vec{v}_2 (\vec{S}_1 \cdot \vec{v}_2)^2 \right) \Bigg\}
\end{aligned}$$

{DiagS1CES2[2, 2, 36],

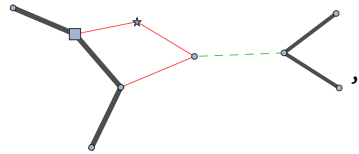

$$\begin{aligned}
& G^2 \left( \frac{1}{r} \left( -\frac{1}{6} \hat{n} \cdot \vec{a}_2 (\hat{n} \cdot \vec{S}_1)^2 - \frac{1}{3} \vec{S}_1 \cdot \vec{a}_2 \hat{n} \cdot \vec{S}_1 - \frac{1}{6} \hat{n} \cdot \vec{S}_1 \hat{n} \cdot \vec{a}_2 \hat{n} \cdot \vec{S}_1 - \frac{7}{6} \hat{n} \cdot \vec{a}_2 \vec{S}_1 \cdot \vec{S}_1 - \frac{1}{6} \hat{n} \cdot \vec{S}_1 \vec{S}_1 \cdot \vec{a}_2 - \frac{7}{6} \hat{n} \cdot \vec{a}_2 \vec{S}_1 \cdot \vec{S}_1 - \right. \right. \\
& \left. \frac{1}{6} \hat{n} \cdot \vec{S}_1 \vec{S}_1 \cdot \vec{a}_2 \right) + \frac{1}{r^2} \left( -\frac{2}{3} (\hat{n} \cdot \vec{v}_2)^2 (\hat{n} \cdot \vec{S}_1)^2 + \frac{1}{3} \hat{n} \cdot \vec{v}_1 \hat{n} \cdot \vec{v}_2 (\hat{n} \cdot \vec{S}_1)^2 - \frac{1}{3} \vec{v}_1 \cdot \vec{v}_2 (\hat{n} \cdot \vec{S}_1)^2 + \right.
\end{aligned}$$









$$\begin{aligned} & 6 \left( \hat{n} \cdot \vec{S}_1 \right)^2 \vec{v}_1 \cdot \vec{v}_2 \left( \hat{n} \cdot \vec{v}_1 \right)^2 - 2 \vec{S}_1 \cdot \vec{S}_1 \vec{v}_1 \cdot \vec{v}_2 \left( \hat{n} \cdot \vec{v}_1 \right)^2 - 2 \left( \hat{n} \cdot \vec{S}_1 \right)^2 \vec{v}_2 \cdot \vec{v}_2 \left( \hat{n} \cdot \vec{v}_1 \right)^2 - \frac{2}{3} \vec{S}_1 \cdot \vec{S}_1 \vec{v}_2 \cdot \vec{v}_2 \left( \hat{n} \cdot \vec{v}_1 \right)^2 + \\ & 6 \hat{n} \cdot \vec{v}_2 \left( \vec{S}_1 \cdot \vec{v}_1 \right)^2 \hat{n} \cdot \vec{v}_1 - 20 \hat{n} \cdot \vec{S}_1 \left( \hat{n} \cdot \vec{v}_2 \right)^2 \vec{S}_1 \cdot \vec{v}_1 \hat{n} \cdot \vec{v}_1 + \frac{20}{3} \hat{n} \cdot \vec{v}_2 \vec{S}_1 \cdot \vec{v}_1 \vec{S}_1 \cdot \vec{v}_2 \hat{n} \cdot \vec{v}_1 - \\ & 6 \left( \hat{n} \cdot \vec{S}_1 \right)^2 \hat{n} \cdot \vec{v}_2 \vec{v}_1 \cdot \vec{v}_1 \hat{n} \cdot \vec{v}_1 - 2 \hat{n} \cdot \vec{v}_2 \vec{S}_1 \cdot \vec{S}_1 \vec{v}_1 \cdot \vec{v}_1 \hat{n} \cdot \vec{v}_1 + 2 \hat{n} \cdot \vec{S}_1 \vec{S}_1 \cdot \vec{v}_2 \vec{v}_1 \cdot \vec{v}_1 \hat{n} \cdot \vec{v}_1 - \\ & 8 \left( \hat{n} \cdot \vec{S}_1 \right)^2 \hat{n} \cdot \vec{v}_2 \vec{v}_1 \cdot \vec{v}_2 \hat{n} \cdot \vec{v}_1 - \frac{8}{3} \hat{n} \cdot \vec{v}_2 \vec{S}_1 \cdot \vec{S}_1 \vec{v}_1 \cdot \vec{v}_2 \hat{n} \cdot \vec{v}_1 + 8 \hat{n} \cdot \vec{S}_1 \vec{S}_1 \cdot \vec{v}_1 \vec{v}_1 \cdot \vec{v}_2 \hat{n} \cdot \vec{v}_1 + \\ & \frac{8}{3} \hat{n} \cdot \vec{S}_1 \vec{S}_1 \cdot \vec{v}_2 \vec{v}_1 \cdot \vec{v}_2 \hat{n} \cdot \vec{v}_1 + \frac{10}{3} \hat{n} \cdot \vec{S}_1 \vec{S}_1 \cdot \vec{v}_1 \vec{v}_2 \cdot \vec{v}_2 \hat{n} \cdot \vec{v}_1 + \frac{8}{3} \left( \hat{n} \cdot \vec{v}_2 \right)^2 \left( \vec{S}_1 \cdot \vec{v}_1 \right)^2 + \\ & \frac{2}{3} \left( \hat{n} \cdot \vec{S}_1 \right)^2 \left( \vec{v}_1 \cdot \vec{v}_2 \right)^2 + \frac{1}{3} \vec{S}_1 \cdot \vec{S}_1 \left( \vec{v}_1 \cdot \vec{v}_2 \right)^2 - 2 \left( \hat{n} \cdot \vec{S}_1 \right)^2 \left( \hat{n} \cdot \vec{v}_2 \right)^2 \vec{v}_1 \cdot \vec{v}_1 - \frac{1}{6} \left( \vec{S}_1 \cdot \vec{v}_2 \right)^2 \vec{v}_1 \cdot \vec{v}_1 - \\ & \frac{2}{3} \left( \hat{n} \cdot \vec{v}_2 \right)^2 \vec{S}_1 \cdot \vec{S}_1 \vec{v}_1 \cdot \vec{v}_1 + 4 \hat{n} \cdot \vec{S}_1 \hat{n} \cdot \vec{v}_2 \vec{S}_1 \cdot \vec{v}_1 \vec{v}_1 \cdot \vec{v}_1 + \frac{4}{3} \hat{n} \cdot \vec{S}_1 \hat{n} \cdot \vec{v}_2 \vec{S}_1 \cdot \vec{v}_2 \vec{v}_1 \cdot \vec{v}_1 - \vec{S}_1 \cdot \vec{v}_1 \vec{S}_1 \cdot \vec{v}_2 \vec{v}_1 \cdot \vec{v}_1 - \\ & \frac{3}{2} \left( \vec{S}_1 \cdot \vec{v}_1 \right)^2 \vec{v}_1 \cdot \vec{v}_2 + \frac{20}{3} \hat{n} \cdot \vec{S}_1 \hat{n} \cdot \vec{v}_2 \vec{S}_1 \cdot \vec{v}_1 \vec{v}_1 \cdot \vec{v}_2 - \frac{5}{3} \vec{S}_1 \cdot \vec{v}_1 \vec{S}_1 \cdot \vec{v}_2 \vec{v}_1 \cdot \vec{v}_2 + \left( \hat{n} \cdot \vec{S}_1 \right)^2 \vec{v}_1 \cdot \vec{v}_1 \vec{v}_1 \cdot \vec{v}_2 + \\ & \left. \frac{1}{2} \vec{S}_1 \cdot \vec{S}_1 \vec{v}_1 \cdot \vec{v}_1 \vec{v}_1 \cdot \vec{v}_2 - \frac{2}{3} \left( \vec{S}_1 \cdot \vec{v}_1 \right)^2 \vec{v}_2 \cdot \vec{v}_2 + \frac{1}{3} \left( \hat{n} \cdot \vec{S}_1 \right)^2 \vec{v}_1 \cdot \vec{v}_1 \vec{v}_2 \cdot \vec{v}_2 + \frac{1}{6} \vec{S}_1 \cdot \vec{S}_1 \vec{v}_1 \cdot \vec{v}_1 \vec{v}_2 \cdot \vec{v}_2 \right) \Bigg) m_2 C_{ES^2_1} \} \end{aligned}$$

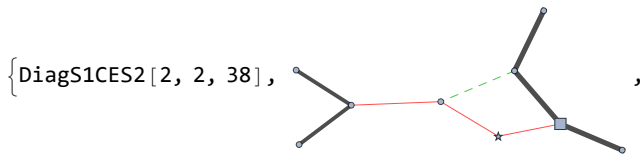

$$\begin{aligned}
G^2 \left( \frac{1}{r} \left( \frac{2}{3} \hat{n} \cdot \vec{a}_1 \left( \hat{n} \cdot \vec{S}_1 \right)^2 - \frac{2}{3} \vec{S}_1 \cdot \vec{a}_1 \hat{n} \cdot \vec{S}_1 + \frac{2}{3} \hat{n} \cdot \vec{S}_1 \hat{n} \cdot \vec{a}_1 \hat{n} \cdot \vec{S}_1 + \right. \right. \\
\left. \left. \frac{8}{3} \hat{n} \cdot \vec{a}_1 \vec{S}_1 \cdot \vec{S}_1 - \frac{1}{3} \hat{n} \cdot \vec{S}_1 \vec{S}_1 \cdot \vec{a}_1 + \frac{8}{3} \hat{n} \cdot \vec{a}_1 \vec{S}_1 \cdot \vec{S}_1 - \frac{1}{3} \hat{n} \cdot \vec{S}_1 \vec{S}_1 \cdot \vec{a}_1 \right) + \frac{1}{r^2} \right. \\
\left( -\frac{2}{3} \left( \hat{n} \cdot \vec{v}_1 \right)^2 \left( \hat{n} \cdot \vec{S}_1 \right)^2 + \frac{8}{3} \hat{n} \cdot \vec{v}_1 \hat{n} \cdot \vec{v}_2 \left( \hat{n} \cdot \vec{S}_1 \right)^2 + \frac{1}{6} \vec{v}_1 \cdot \vec{v}_1 \left( \hat{n} \cdot \vec{S}_1 \right)^2 - \frac{2}{3} \vec{v}_1 \cdot \vec{v}_2 \left( \hat{n} \cdot \vec{S}_1 \right)^2 - 4 \hat{n} \cdot \vec{a}_1 \hat{n} \cdot \vec{S}_1 \hat{n} \cdot \vec{v}_1 \right. \\
\left. \hat{n} \cdot \vec{S}_1 - 2 \hat{n} \cdot \vec{a}_2 \hat{n} \cdot \vec{S}_1 \hat{n} \cdot \vec{v}_1 \hat{n} \cdot \vec{S}_1 - 2 \hat{n} \cdot \vec{a}_1 \hat{n} \cdot \vec{S}_1 \hat{n} \cdot \vec{v}_2 \hat{n} \cdot \vec{S}_1 - \frac{1}{3} \hat{n} \cdot \vec{v}_1 \vec{S}_1 \cdot \vec{v}_1 \hat{n} \cdot \vec{S}_1 - \frac{4}{3} \hat{n} \cdot \vec{v}_2 \vec{S}_1 \cdot \vec{v}_1 \hat{n} \cdot \vec{S}_1 - \right. \\
\left. \frac{4}{3} \hat{n} \cdot \vec{v}_1 \vec{S}_1 \cdot \vec{v}_2 \hat{n} \cdot \vec{S}_1 + \frac{1}{2} \hat{n} \cdot \vec{S}_1 \vec{a}_1 \cdot \vec{v}_2 \hat{n} \cdot \vec{S}_1 + \hat{n} \cdot \vec{v}_1 \vec{S}_1 \cdot \vec{a}_1 \hat{n} \cdot \vec{S}_1 + \hat{n} \cdot \vec{v}_2 \vec{S}_1 \cdot \vec{a}_1 \hat{n} \cdot \vec{S}_1 + \frac{1}{2} \hat{n} \cdot \vec{v}_1 \vec{S}_1 \cdot \vec{a}_2 \hat{n} \cdot \vec{S}_1 + \right. \\
\left. 2 \hat{n} \cdot \vec{a}_1 \vec{S}_1 \cdot \vec{v}_1 \hat{n} \cdot \vec{S}_1 + \hat{n} \cdot \vec{a}_2 \vec{S}_1 \cdot \vec{v}_1 \hat{n} \cdot \vec{S}_1 + \frac{1}{2} \hat{n} \cdot \vec{a}_1 \vec{S}_1 \cdot \vec{v}_2 \hat{n} \cdot \vec{S}_1 + \hat{n} \cdot \vec{S}_1 \vec{v}_1 \cdot \vec{a}_1 \hat{n} \cdot \vec{S}_1 + \frac{1}{2} \hat{n} \cdot \vec{S}_1 \vec{v}_1 \cdot \vec{a}_2 \hat{n} \cdot \vec{S}_1 - \right. \\
\left( \hat{n} \cdot \vec{a}_1 \right)^2 \left( \hat{n} \cdot \vec{S}_1 \right)^2 - \frac{2}{3} \hat{n} \cdot \vec{S}_1 \hat{n} \cdot \vec{S}_1 \left( \hat{n} \cdot \vec{v}_1 \right)^2 + \frac{1}{3} \left( \vec{S}_1 \cdot \vec{v}_1 \right)^2 - \frac{1}{2} \left( \vec{S}_1 \cdot \vec{a}_1 \right)^2 + \frac{8}{3} \hat{n} \cdot \vec{S}_1 \hat{n} \cdot \vec{S}_1 \hat{n} \cdot \vec{v}_1 \hat{n} \cdot \vec{v}_2 - \\
\frac{7}{3} \left( \hat{n} \cdot \vec{v}_1 \right)^2 \vec{S}_1 \cdot \vec{S}_1 + \frac{16}{3} \hat{n} \cdot \vec{v}_1 \hat{n} \cdot \vec{v}_2 \vec{S}_1 \cdot \vec{S}_1 + \hat{n} \cdot \vec{S}_1 \hat{n} \cdot \vec{v}_1 \vec{S}_1 \cdot \vec{a}_1 + \hat{n} \cdot \vec{S}_1 \hat{n} \cdot \vec{v}_2 \vec{S}_1 \cdot \vec{a}_1 + \frac{1}{2} \hat{n} \cdot \vec{S}_1 \hat{n} \cdot \vec{v}_1 \vec{S}_1 \cdot \vec{a}_2 + \\
2 \hat{n} \cdot \vec{a}_1 \hat{n} \cdot \vec{S}_1 \vec{S}_1 \cdot \vec{v}_1 + \hat{n} \cdot \vec{a}_2 \hat{n} \cdot \vec{S}_1 \vec{S}_1 \cdot \vec{v}_1 + \frac{1}{2} \hat{n} \cdot \vec{a}_1 \hat{n} \cdot \vec{S}_1 \vec{S}_1 \cdot \vec{v}_2 + \frac{2}{3} \vec{S}_1 \cdot \vec{v}_1 \vec{S}_1 \cdot \vec{v}_2 - \frac{1}{6} \hat{n} \cdot \vec{S}_1 \hat{n} \cdot \vec{v}_1 \vec{S}_1^2 \cdot \vec{v}_1 - \\
\frac{2}{3} \hat{n} \cdot \vec{S}_1 \hat{n} \cdot \vec{v}_2 \vec{S}_1 \cdot \vec{v}_1 - \frac{2}{3} \hat{n} \cdot \vec{S}_1 \hat{n} \cdot \vec{v}_1 \vec{S}_1 \cdot \vec{v}_2 + \frac{1}{4} \left( \hat{n} \cdot \vec{S}_1 \right)^2 \vec{a}_1 \cdot \vec{a}_1 - 6 \hat{n} \cdot \vec{a}_1 \hat{n} \cdot \vec{v}_1 \vec{S}_1 \cdot \vec{S}_1 - 3 \hat{n} \cdot \vec{a}_2 \hat{n} \cdot \vec{v}_1 \vec{S}_1 \cdot \vec{S}_1 - \\
3 \hat{n} \cdot \vec{a}_1 \hat{n} \cdot \vec{v}_2 \vec{S}_1 \cdot \vec{S}_1 + \frac{3}{2} \vec{a}_1 \cdot \vec{v}_2 \vec{S}_1 \cdot \vec{S}_1 - \frac{7}{3} \left( \hat{n} \cdot \vec{v}_1 \right)^2 \vec{S}_1 \cdot \vec{S}_1 + \frac{16}{3} \hat{n} \cdot \vec{v}_1 \hat{n} \cdot \vec{v}_2 \vec{S}_1 \cdot \vec{S}_1 + \frac{3}{2} \hat{n} \cdot \vec{a}_1 \hat{n} \cdot \vec{S}_1 \vec{S}_1 \cdot \vec{a}_1 - \\
\frac{1}{\vec{S}_1 \cdot \vec{v}_1 \vec{S}_1 \cdot \vec{a}_1} - \frac{1}{2} \vec{S}_1 \cdot \vec{v}_2 \vec{S}_1 \cdot \vec{a}_1 - \frac{1}{2} \vec{S}_1 \cdot \vec{v}_1 \vec{S}_1 \cdot \vec{a}_2 - \frac{3}{2} \left( \hat{n} \cdot \vec{a}_1 \right)^2 \vec{S}_1 \cdot \vec{S}_1 + \frac{3}{4} \vec{a}_1 \cdot \vec{a}_1 \vec{S}_1 \cdot \vec{S}_1 - \frac{1}{6} \hat{n} \cdot \vec{S}_1 \hat{n} \cdot \vec{v}_1 \vec{S}_1 \cdot \vec{v}_1 - \\
\frac{2}{3} \hat{n} \cdot \vec{S}_1 \hat{n} \cdot \vec{v}_2 \vec{S}_1 \cdot \vec{v}_1 - \vec{S}_1 \cdot \vec{a}_1 \vec{S}_1 \cdot \vec{v}_1 - \frac{1}{2} \vec{S}_1 \cdot \vec{a}_2 \vec{S}_1 \cdot \vec{v}_1 + \frac{1}{3} \vec{S}_1 \cdot \vec{v}_1 \vec{S}_1 \cdot \vec{v}_1 + \frac{1}{3} \vec{S}_1 \cdot \vec{v}_2 \vec{S}_1 \cdot \vec{v}_1 - \frac{2}{3} \hat{n} \cdot \vec{S}_1 \hat{n} \cdot \vec{v}_1 \vec{S}_1 \cdot \vec{v}_2 - \\
\frac{1}{2} \vec{S}_1 \cdot \vec{a}_1 \vec{S}_1 \cdot \vec{v}_2 + \frac{1}{3} \vec{S}_1 \cdot \vec{v}_1 \vec{S}_1 \cdot \vec{v}_2 + 3 \vec{S}_1 \cdot \vec{S}_1 \vec{v}_1 \cdot \vec{a}_1 + \frac{3}{2} \vec{S}_1 \cdot \vec{S}_1 \vec{v}_1 \cdot \vec{a}_2 + \frac{1}{6} \hat{n} \cdot \vec{S}_1 \hat{n} \cdot \vec{S}_1 \vec{v}_1 \cdot \vec{v}_1 +
\end{aligned}$$

$$\begin{aligned}
& \frac{7}{6} \frac{1}{S_1} \cdot \frac{1}{S_1} \vec{v}_1 \cdot \vec{v}_1 + \frac{7}{6} \vec{S}_1 \cdot \frac{2}{S_1} \vec{v}_1 \cdot \vec{v}_1 - \frac{2}{3} \hat{n} \cdot \frac{2}{S_1} \hat{n} \cdot \vec{S}_1 \vec{v}_1 \cdot \vec{v}_2 - \frac{8}{3} \frac{1}{S_1} \cdot \frac{1}{S_1} \vec{v}_1 \cdot \vec{v}_2 - \frac{8}{3} \vec{S}_1 \cdot \frac{2}{S_1} \vec{v}_1 \cdot \vec{v}_2 \Big) + \frac{1}{r^3} \\
& \left( 4 \hat{n} \cdot \frac{1}{S_1} \hat{n} \cdot \vec{S}_1 (\hat{n} \cdot \vec{v}_1)^3 + \frac{16}{3} \vec{S}_1 \cdot \frac{1}{S_1} (\hat{n} \cdot \vec{v}_1)^3 + 6 \hat{n} \cdot \vec{a}_1 (\hat{n} \cdot \vec{S}_1)^2 (\hat{n} \cdot \vec{v}_1)^2 + 5 \hat{n} \cdot \vec{a}_2 (\hat{n} \cdot \vec{S}_1)^2 (\hat{n} \cdot \vec{v}_1)^2 - \right. \\
& 22 \hat{n} \cdot \frac{1}{S_1} \hat{n} \cdot \vec{S}_1 \hat{n} \cdot \vec{v}_2 (\hat{n} \cdot \vec{v}_1)^2 - 2 \hat{n} \cdot \vec{S}_1 \frac{1}{S_1} \cdot \vec{v}_1 (\hat{n} \cdot \vec{v}_1)^2 + \frac{11}{3} \hat{n} \cdot \vec{S}_1 \frac{1}{S_1} \cdot \vec{v}_2 (\hat{n} \cdot \vec{v}_1)^2 - \frac{64}{3} \hat{n} \cdot \vec{v}_2 \vec{S}_1 \cdot \frac{1}{S_1} (\hat{n} \cdot \vec{v}_1)^2 - \\
& 3 \hat{n} \cdot \vec{S}_1 \vec{S}_1 \cdot \vec{a}_1 (\hat{n} \cdot \vec{v}_1)^2 - \frac{5}{3} \hat{n} \cdot \vec{S}_1 \vec{S}_1 \cdot \vec{a}_2 (\hat{n} \cdot \vec{v}_1)^2 + 6 \hat{n} \cdot \vec{a}_1 \vec{S}_1 \cdot \vec{S}_1 (\hat{n} \cdot \vec{v}_1)^2 + \frac{14}{3} \hat{n} \cdot \vec{a}_2 \vec{S}_1 \cdot \vec{S}_1 (\hat{n} \cdot \vec{v}_1)^2 - \\
& 2 \hat{n} \cdot \frac{1}{S_1} \vec{S}_1 \cdot \vec{v}_1 (\hat{n} \cdot \vec{v}_1)^2 + \frac{11}{3} \hat{n} \cdot \frac{1}{S_1} \vec{S}_1 \cdot \vec{v}_2 (\hat{n} \cdot \vec{v}_1)^2 - 12 \hat{n} \cdot \frac{1}{S_1} \hat{n} \cdot \vec{S}_1 (\hat{n} \cdot \vec{v}_2)^2 \hat{n} \cdot \vec{v}_1 - \hat{n} \cdot \vec{a}_1 (\hat{n} \cdot \vec{S}_1)^2 \hat{n} \cdot \vec{v}_2 \hat{n} \cdot \vec{v}_1 + \\
& \frac{34}{3} \hat{n} \cdot \vec{S}_1 \hat{n} \cdot \vec{v}_2 \frac{1}{S_1} \cdot \vec{v}_1 \hat{n} \cdot \vec{v}_1 + 4 \hat{n} \cdot \vec{S}_1 \hat{n} \cdot \vec{v}_2 \frac{1}{S_1} \cdot \vec{v}_2 \hat{n} \cdot \vec{v}_1 + \frac{1}{6} (\hat{n} \cdot \vec{S}_1)^2 \vec{a}_1 \cdot \vec{v}_2 \hat{n} \cdot \vec{v}_1 - 12 (\hat{n} \cdot \vec{v}_2)^2 \vec{S}_1 \cdot \frac{1}{S_1} \hat{n} \cdot \vec{v}_1 + \\
& \frac{4}{3} \hat{n} \cdot \vec{S}_1 \hat{n} \cdot \vec{v}_2 \vec{S}_1 \cdot \vec{a}_1 \hat{n} \cdot \vec{v}_1 - \frac{4}{3} \hat{n} \cdot \vec{a}_1 \hat{n} \cdot \vec{v}_2 \vec{S}_1 \cdot \vec{S}_1 \hat{n} \cdot \vec{v}_1 + \frac{1}{3} \vec{a}_1 \cdot \vec{v}_2 \vec{S}_1 \cdot \vec{S}_1 \hat{n} \cdot \vec{v}_1 - 5 \hat{n} \cdot \vec{a}_1 \hat{n} \cdot \vec{S}_1 \vec{S}_1 \cdot \vec{v}_1 \hat{n} \cdot \vec{v}_1 - \\
& \frac{16}{3} \hat{n} \cdot \vec{a}_2 \hat{n} \cdot \vec{S}_1 \vec{S}_1 \cdot \vec{v}_1 \hat{n} \cdot \vec{v}_1 + \frac{34}{3} \hat{n} \cdot \frac{1}{S_1} \hat{n} \cdot \vec{v}_2 \vec{S}_1 \cdot \vec{v}_1 \hat{n} \cdot \vec{v}_1 + 2 \frac{1}{S_1} \cdot \vec{v}_1 \vec{S}_1 \cdot \vec{v}_1 \hat{n} \cdot \vec{v}_1 - \frac{17}{6} \frac{1}{S_1} \cdot \vec{v}_2 \vec{S}_1 \cdot \vec{v}_1 \hat{n} \cdot \vec{v}_1 + \\
& 2 \vec{S}_1 \cdot \vec{a}_1 \vec{S}_1 \cdot \vec{v}_1 \hat{n} \cdot \vec{v}_1 + \frac{4}{3} \vec{S}_1 \cdot \vec{a}_2 \vec{S}_1 \cdot \vec{v}_1 \hat{n} \cdot \vec{v}_1 + \frac{1}{3} \hat{n} \cdot \vec{a}_1 \hat{n} \cdot \vec{S}_1 \vec{S}_1 \cdot \vec{v}_2 \hat{n} \cdot \vec{v}_1 + 4 \hat{n} \cdot \frac{1}{S_1} \hat{n} \cdot \vec{v}_2 \vec{S}_1 \cdot \vec{v}_2 \hat{n} \cdot \vec{v}_1 - \\
& \frac{17}{6} \frac{1}{S_1} \cdot \vec{v}_1 \vec{S}_1 \cdot \vec{v}_2 \hat{n} \cdot \vec{v}_1 - \frac{1}{S_1} \cdot \vec{v}_2 \vec{S}_1 \cdot \vec{v}_2 \hat{n} \cdot \vec{v}_1 - \frac{1}{3} \vec{S}_1 \cdot \vec{a}_1 \vec{S}_1 \cdot \vec{v}_2 \hat{n} \cdot \vec{v}_1 - \frac{3}{2} (\hat{n} \cdot \vec{S}_1)^2 \vec{v}_1 \cdot \vec{a}_1 \hat{n} \cdot \vec{v}_1 - \\
& \frac{7}{2} \vec{S}_1 \cdot \vec{S}_1 \vec{v}_1 \cdot \vec{a}_1 \hat{n} \cdot \vec{v}_1 - \frac{5}{3} (\hat{n} \cdot \vec{S}_1)^2 \vec{v}_1 \cdot \vec{a}_2 \hat{n} \cdot \vec{v}_1 - \frac{7}{3} \vec{S}_1 \cdot \vec{S}_1 \vec{v}_1 \cdot \vec{a}_2 \hat{n} \cdot \vec{v}_1 - 6 \vec{S}_1 \cdot \frac{1}{S_1} \vec{v}_1 \cdot \vec{v}_1 \hat{n} \cdot \vec{v}_1 + \\
& \frac{22}{3} \hat{n} \cdot \frac{1}{S_1} \hat{n} \cdot \vec{S}_1 \vec{v}_1 \cdot \vec{v}_2 \hat{n} \cdot \vec{v}_1 + \frac{32}{3} \vec{S}_1 \cdot \frac{1}{S_1} \vec{v}_1 \cdot \vec{v}_2 \hat{n} \cdot \vec{v}_1 + 2 \hat{n} \cdot \frac{1}{S_1} \hat{n} \cdot \vec{S}_1 \vec{v}_2 \cdot \vec{v}_2 \hat{n} \cdot \vec{v}_1 + 3 \vec{S}_1 \cdot \frac{1}{S_1} \vec{v}_2 \cdot \vec{v}_2 \hat{n} \cdot \vec{v}_1 + \\
& \frac{1}{2} \hat{n} \cdot \vec{a}_1 (\vec{S}_1 \cdot \vec{v}_1)^2 + \frac{2}{3} \hat{n} \cdot \vec{a}_2 (\vec{S}_1 \cdot \vec{v}_1)^2 + 4 \hat{n} \cdot \vec{S}_1 (\hat{n} \cdot \vec{v}_2)^2 \frac{1}{S_1} \cdot \vec{v}_1 + 4 \hat{n} \cdot \frac{1}{S_1} (\hat{n} \cdot \vec{v}_2)^2 \vec{S}_1 \cdot \vec{v}_1 - \\
& \frac{2}{3} \hat{n} \cdot \vec{a}_1 \hat{n} \cdot \vec{S}_1 \hat{n} \cdot \vec{v}_2 \vec{S}_1 \cdot \vec{v}_1 - \frac{10}{3} \hat{n} \cdot \vec{v}_2 \frac{1}{S_1} \cdot \vec{v}_1 \vec{S}_1 \cdot \vec{v}_1 - 2 \hat{n} \cdot \vec{v}_2 \frac{1}{S_1} \cdot \vec{v}_2 \vec{S}_1 \cdot \vec{v}_1 + \frac{1}{6} \hat{n} \cdot \vec{S}_1 \vec{a}_1 \cdot \vec{v}_2 \vec{S}_1 \cdot \vec{v}_1 - \\
& \frac{1}{3} \hat{n} \cdot \vec{v}_2 \vec{S}_1 \cdot \vec{a}_1 \vec{S}_1 \cdot \vec{v}_1 - 2 \hat{n} \cdot \vec{v}_2 \frac{1}{S_1} \cdot \vec{v}_1 \vec{S}_1 \cdot \vec{v}_2 + \frac{1}{6} \hat{n} \cdot \vec{a}_1 \vec{S}_1 \cdot \vec{v}_1 \vec{S}_1 \cdot \vec{v}_2 - \frac{1}{3} (\hat{n} \cdot \vec{S}_1)^2 \hat{n} \cdot \vec{v}_2 \vec{v}_1 \cdot \vec{a}_1 + \\
& \frac{5}{6} \hat{n} \cdot \vec{v}_2 \vec{S}_1 \cdot \vec{S}_1 \vec{v}_1 \cdot \vec{a}_1 + \hat{n} \cdot \vec{S}_1 \vec{S}_1 \cdot \vec{v}_1 \vec{v}_1 \cdot \vec{a}_1 + \frac{1}{6} \hat{n} \cdot \vec{S}_1 \vec{S}_1 \cdot \vec{v}_2 \vec{v}_1 \cdot \vec{a}_1 + \frac{4}{3} \hat{n} \cdot \vec{S}_1 \vec{S}_1 \cdot \vec{v}_1 \vec{v}_1 \cdot \vec{a}_2 - \\
& \frac{3}{2} \hat{n} \cdot \vec{a}_1 (\hat{n} \cdot \vec{S}_1)^2 \vec{v}_1 \cdot \vec{v}_1 - \frac{4}{3} \hat{n} \cdot \vec{a}_2 (\hat{n} \cdot \vec{S}_1)^2 \vec{v}_1 \cdot \vec{v}_1 + \frac{14}{3} \hat{n} \cdot \frac{1}{S_1} \hat{n} \cdot \vec{S}_1 \hat{n} \cdot \vec{v}_2 \vec{v}_1 \cdot \vec{v}_1 - \frac{7}{6} \hat{n} \cdot \vec{S}_1 \frac{1}{S_1} \cdot \vec{v}_2 \vec{v}_1 \cdot \vec{v}_1 + \\
& \frac{13}{3} \hat{n} \cdot \vec{v}_2 \vec{S}_1 \cdot \frac{1}{S_1} \vec{v}_1 \cdot \vec{v}_1 + \hat{n} \cdot \vec{S}_1 \vec{S}_1 \cdot \vec{a}_1 \vec{v}_1 \cdot \vec{v}_1 + \frac{2}{3} \hat{n} \cdot \vec{S}_1 \vec{S}_1 \cdot \vec{a}_2 \vec{v}_1 \cdot \vec{v}_1 - \hat{n} \cdot \vec{a}_1 \vec{S}_1 \cdot \vec{S}_1 \vec{v}_1 \cdot \vec{v}_1 - \\
& \frac{2}{3} \hat{n} \cdot \vec{a}_2 \vec{S}_1 \cdot \vec{S}_1 \vec{v}_1 \cdot \vec{v}_1 - \frac{7}{6} \hat{n} \cdot \frac{1}{S_1} \vec{S}_1 \cdot \vec{v}_2 \vec{v}_1 \cdot \vec{v}_1 + \frac{1}{6} \hat{n} \cdot \vec{a}_1 (\hat{n} \cdot \vec{S}_1)^2 \vec{v}_1 \cdot \vec{v}_2 + 4 \hat{n} \cdot \frac{1}{S_1} \hat{n} \cdot \vec{S}_1 \hat{n} \cdot \vec{v}_2 \vec{v}_1 \cdot \vec{v}_2 - \\
& \frac{17}{6} \hat{n} \cdot \vec{S}_1 \frac{1}{S_1} \cdot \vec{v}_1 \vec{v}_1 \cdot \vec{v}_2 - \hat{n} \cdot \vec{S}_1 \frac{1}{S_1} \cdot \vec{v}_2 \vec{v}_1 \cdot \vec{v}_2 + 6 \hat{n} \cdot \vec{v}_2 \vec{S}_1 \cdot \frac{1}{S_1} \vec{v}_1 \cdot \vec{v}_2 - \frac{1}{3} \hat{n} \cdot \vec{S}_1 \vec{S}_1 \cdot \vec{a}_1 \vec{v}_1 \cdot \vec{v}_2 + \\
& \frac{1}{3} \hat{n} \cdot \vec{a}_1 \vec{S}_1 \cdot \vec{S}_1 \vec{v}_1 \cdot \vec{v}_2 - \frac{17}{6} \hat{n} \cdot \frac{1}{S_1} \vec{S}_1 \cdot \vec{v}_1 \vec{v}_1 \cdot \vec{v}_2 - \hat{n} \cdot \frac{1}{S_1} \vec{S}_1 \cdot \vec{v}_2 \vec{v}_1 \cdot \vec{v}_2 - \hat{n} \cdot \vec{S}_1 \frac{1}{S_1} \cdot \vec{v}_1 \vec{v}_2 \cdot \vec{v}_2 - \hat{n} \cdot \vec{S}_1 \frac{1}{S_1} \cdot \vec{v}_1 \vec{v}_2 \cdot \vec{v}_2 \Big) + \\
& \frac{1}{r^4} \left( -5 (\hat{n} \cdot \vec{S}_1)^2 (\hat{n} \cdot \vec{v}_1)^4 - \frac{17}{4} \vec{S}_1 \cdot \vec{S}_1 (\hat{n} \cdot \vec{v}_1)^4 + 35 (\hat{n} \cdot \vec{S}_1)^2 \hat{n} \cdot \vec{v}_2 (\hat{n} \cdot \vec{v}_1)^3 + \frac{95}{4} \hat{n} \cdot \vec{v}_2 \vec{S}_1 \cdot \vec{S}_1 (\hat{n} \cdot \vec{v}_1)^3 + \right. \\
& \frac{23}{4} \hat{n} \cdot \vec{S}_1 \vec{S}_1 \cdot \vec{v}_1 (\hat{n} \cdot \vec{v}_1)^3 - \frac{35}{4} \hat{n} \cdot \vec{S}_1 \vec{S}_1 \cdot \vec{v}_2 (\hat{n} \cdot \vec{v}_1)^3 + 40 (\hat{n} \cdot \vec{S}_1)^2 (\hat{n} \cdot \vec{v}_2)^2 (\hat{n} \cdot \vec{v}_1)^2 - \\
& \frac{7}{4} (\vec{S}_1 \cdot \vec{v}_1)^2 (\hat{n} \cdot \vec{v}_1)^2 + \frac{5}{3} (\vec{S}_1 \cdot \vec{v}_2)^2 (\hat{n} \cdot \vec{v}_1)^2 + 28 (\hat{n} \cdot \vec{v}_2)^2 \vec{S}_1 \cdot \vec{S}_1 (\hat{n} \cdot \vec{v}_1)^2 - \\
& \frac{75}{2} \hat{n} \cdot \vec{S}_1 \hat{n} \cdot \vec{v}_2 \vec{S}_1 \cdot \vec{v}_1 (\hat{n} \cdot \vec{v}_1)^2 - 20 \hat{n} \cdot \vec{S}_1 \hat{n} \cdot \vec{v}_2 \vec{S}_1 \cdot \vec{v}_2 (\hat{n} \cdot \vec{v}_1)^2 + \frac{25}{4} \vec{S}_1 \cdot \vec{v}_1 \vec{S}_1 \cdot \vec{v}_2 (\hat{n} \cdot \vec{v}_1)^2 + \\
& \left. \frac{9}{8} (\hat{n} \cdot \vec{S}_1)^2 \vec{v}_1 \cdot \vec{v}_1 (\hat{n} \cdot \vec{v}_1)^2 + \frac{45}{8} \vec{S}_1 \cdot \vec{S}_1 \vec{v}_1 \cdot \vec{v}_1 (\hat{n} \cdot \vec{v}_1)^2 - \frac{105}{8} (\hat{n} \cdot \vec{S}_1)^2 \vec{v}_1 \cdot \vec{v}_2 (\hat{n} \cdot \vec{v}_1)^2 - \right)
\end{aligned}$$

$$\begin{aligned}
& \frac{95}{8} \vec{S}_1 \cdot \vec{S}_1 \vec{v}_1 \cdot \vec{v}_2 (\hat{n} \cdot \vec{v}_1)^2 - 5 (\hat{n} \cdot \vec{S}_1)^2 \vec{v}_2 \cdot \vec{v}_2 (\hat{n} \cdot \vec{v}_1)^2 - \frac{14}{3} \vec{S}_1 \cdot \vec{S}_1 \vec{v}_2 \cdot \vec{v}_2 (\hat{n} \cdot \vec{v}_1)^2 + \\
& 7 \hat{n} \cdot \vec{v}_2 (\vec{S}_1 \cdot \vec{v}_1)^2 \hat{n} \cdot \vec{v}_1 - 32 \hat{n} \cdot \vec{S}_1 (\hat{n} \cdot \vec{v}_2)^2 \vec{S}_1 \cdot \vec{v}_1 \hat{n} \cdot \vec{v}_1 + \frac{32}{3} \hat{n} \cdot \vec{v}_2 \vec{S}_1 \cdot \vec{v}_1 \vec{S}_1 \cdot \vec{v}_2 \hat{n} \cdot \vec{v}_1 - \\
& \frac{75}{4} (\hat{n} \cdot \vec{S}_1)^2 \hat{n} \cdot \vec{v}_2 \vec{v}_1 \cdot \vec{v}_1 \hat{n} \cdot \vec{v}_1 - \frac{17}{2} \hat{n} \cdot \vec{v}_2 \vec{S}_1 \cdot \vec{S}_1 \vec{v}_1 \cdot \vec{v}_1 \hat{n} \cdot \vec{v}_1 - \frac{9}{4} \hat{n} \cdot \vec{S}_1 \vec{S}_1 \cdot \vec{v}_1 \vec{v}_1 \cdot \vec{v}_1 \hat{n} \cdot \vec{v}_1 + \\
& \frac{25}{4} \hat{n} \cdot \vec{S}_1 \vec{S}_1 \cdot \vec{v}_2 \vec{v}_1 \cdot \vec{v}_1 \hat{n} \cdot \vec{v}_1 - 20 (\hat{n} \cdot \vec{S}_1)^2 \hat{n} \cdot \vec{v}_2 \vec{v}_1 \cdot \vec{v}_2 \hat{n} \cdot \vec{v}_1 - \frac{56}{3} \hat{n} \cdot \vec{v}_2 \vec{S}_1 \cdot \vec{S}_1 \vec{v}_1 \cdot \vec{v}_2 \hat{n} \cdot \vec{v}_1 + \\
& \frac{25}{2} \hat{n} \cdot \vec{S}_1 \vec{S}_1 \cdot \vec{v}_1 \vec{v}_1 \cdot \vec{v}_2 \hat{n} \cdot \vec{v}_1 + \frac{20}{3} \hat{n} \cdot \vec{S}_1 \vec{S}_1 \cdot \vec{v}_2 \vec{v}_1 \cdot \vec{v}_2 \hat{n} \cdot \vec{v}_1 + \frac{16}{3} \hat{n} \cdot \vec{S}_1 \vec{S}_1 \cdot \vec{v}_1 \vec{v}_2 \cdot \vec{v}_2 \hat{n} \cdot \vec{v}_1 + \\
& \frac{8}{3} (\hat{n} \cdot \vec{v}_2)^2 (\vec{S}_1 \cdot \vec{v}_1)^2 + \frac{1}{8} (\hat{n} \cdot \vec{S}_1)^2 (\vec{v}_1 \cdot \vec{v}_1)^2 - \frac{7}{8} \vec{S}_1 \cdot \vec{S}_1 (\vec{v}_1 \cdot \vec{v}_1)^2 + \frac{5}{3} (\hat{n} \cdot \vec{S}_1)^2 (\vec{v}_1 \cdot \vec{v}_2)^2 + \\
& \frac{7}{3} \vec{S}_1 \cdot \vec{S}_1 (\vec{v}_1 \cdot \vec{v}_2)^2 - 8 (\hat{n} \cdot \vec{S}_1)^2 (\hat{n} \cdot \vec{v}_2)^2 \vec{v}_1 \cdot \vec{v}_1 + \frac{1}{2} (\vec{S}_1 \cdot \vec{v}_1)^2 \vec{v}_1 \cdot \vec{v}_1 - \frac{2}{3} (\vec{S}_1 \cdot \vec{v}_2)^2 \vec{v}_1 \cdot \vec{v}_1 - \\
& \frac{8}{3} (\hat{n} \cdot \vec{v}_2)^2 \vec{S}_1 \cdot \vec{S}_1 \vec{v}_1 \cdot \vec{v}_1 + 7 \hat{n} \cdot \vec{S}_1 \hat{n} \cdot \vec{v}_2 \vec{S}_1 \cdot \vec{v}_1 \vec{v}_1 \cdot \vec{v}_1 + \frac{16}{3} \hat{n} \cdot \vec{S}_1 \hat{n} \cdot \vec{v}_2 \vec{S}_1 \cdot \vec{v}_2 \vec{v}_1 \cdot \vec{v}_1 - \frac{7}{4} \vec{S}_1 \cdot \vec{v}_1 \vec{S}_1 \cdot \vec{v}_2 \vec{v}_1 \cdot \vec{v}_1 - \\
& \frac{7}{4} (\vec{S}_1 \cdot \vec{v}_1)^2 \vec{v}_1 \cdot \vec{v}_2 + \frac{32}{3} \hat{n} \cdot \vec{S}_1 \hat{n} \cdot \vec{v}_2 \vec{S}_1 \cdot \vec{v}_1 \vec{v}_1 \cdot \vec{v}_2 - \frac{8}{3} \vec{S}_1 \cdot \vec{v}_1 \vec{S}_1 \cdot \vec{v}_2 \vec{v}_1 \cdot \vec{v}_2 + \frac{25}{8} (\hat{n} \cdot \vec{S}_1)^2 \vec{v}_1 \cdot \vec{v}_1 \vec{v}_1 \cdot \vec{v}_2 + \\
& \frac{17}{8} \vec{S}_1 \cdot \vec{S}_1 \vec{v}_1 \cdot \vec{v}_1 \vec{v}_1 \cdot \vec{v}_2 - \frac{2}{3} (\vec{S}_1 \cdot \vec{v}_1)^2 \vec{v}_2 \cdot \vec{v}_2 + \frac{4}{3} (\hat{n} \cdot \vec{S}_1)^2 \vec{v}_1 \cdot \vec{v}_1 \vec{v}_2 \cdot \vec{v}_2 + \frac{2}{3} \vec{S}_1 \cdot \vec{S}_1 \vec{v}_1 \cdot \vec{v}_1 \vec{v}_2 \cdot \vec{v}_2 \Big) m_2 C_{ES^2_1} \Big\}
\end{aligned}$$

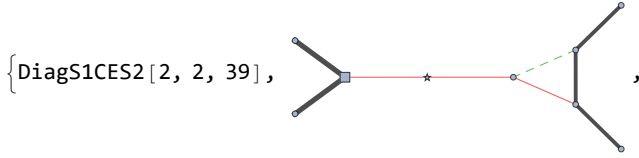

$$\begin{aligned}
& \frac{1}{m_1} G^2 \left( \frac{1}{r} \left( \frac{4}{3} \hat{n} \cdot \vec{a}_2 (\hat{n} \cdot \vec{S}_1)^2 - \frac{4}{3} \vec{S}_1 \cdot \vec{a}_2 \hat{n} \cdot \vec{S}_1 + \frac{4}{3} \hat{n} \cdot \vec{S}_1 \hat{n} \cdot \vec{a}_2 \hat{n} \cdot \vec{S}_1 + \right. \right. \\
& \left. \frac{4}{3} \hat{n} \cdot \vec{a}_2 \vec{S}_1 \cdot \vec{S}_1 - \frac{2}{3} \hat{n} \cdot \vec{S}_1 \vec{S}_1 \cdot \vec{a}_2 + \frac{4}{3} \hat{n} \cdot \vec{a}_2 \vec{S}_1 \cdot \vec{S}_1 - \frac{2}{3} \hat{n} \cdot \vec{S}_1 \vec{S}_1 \cdot \vec{a}_2 \right) + \frac{1}{r^2} \\
& \left( \frac{16}{3} (\hat{n} \cdot \vec{v}_2)^2 \left( (\hat{n} \cdot \vec{S}_1)^2 - \frac{4}{3} \vec{v}_2 \cdot \vec{v}_2 (\hat{n} \cdot \vec{S}_1)^2 - \frac{32}{3} \hat{n} \cdot \vec{a}_2 \hat{n} \cdot \vec{S}_1 \hat{n} \cdot \vec{v}_1 \hat{n} \cdot \vec{S}_1 - \frac{32}{3} \hat{n} \cdot \vec{a}_2 \hat{n} \cdot \vec{S}_1 \hat{n} \cdot \vec{v}_2 \hat{n} \cdot \vec{S}_1 - \right. \right. \\
& \frac{16}{3} \hat{n} \cdot \vec{v}_2 \vec{S}_1 \cdot \vec{v}_2 \hat{n} \cdot \vec{S}_1 + \frac{8}{3} \hat{n} \cdot \vec{v}_1 \vec{S}_1 \cdot \vec{a}_2 \hat{n} \cdot \vec{S}_1 + \frac{8}{3} \hat{n} \cdot \vec{v}_2 \vec{S}_1 \cdot \vec{a}_2 \hat{n} \cdot \vec{S}_1 + \frac{8}{3} \hat{n} \cdot \vec{a}_2 \vec{S}_1 \cdot \vec{v}_1 \hat{n} \cdot \vec{S}_1 + \\
& \frac{8}{3} \hat{n} \cdot \vec{a}_2 \vec{S}_1 \cdot \vec{v}_2 \hat{n} \cdot \vec{S}_1 + \frac{8}{3} \hat{n} \cdot \vec{S}_1 \vec{v}_1 \cdot \vec{a}_2 \hat{n} \cdot \vec{S}_1 + \frac{8}{3} \hat{n} \cdot \vec{S}_1 \vec{v}_2 \cdot \vec{a}_2 \hat{n} \cdot \vec{S}_1 - \frac{8}{3} \hat{n} \cdot \vec{a}_1 \hat{n} \cdot \vec{a}_2 (\hat{n} \cdot \vec{S}_1)^2 + \\
& \frac{16}{3} \hat{n} \cdot \vec{S}_1 \hat{n} \cdot \vec{S}_1 (\hat{n} \cdot \vec{v}_2)^2 + \frac{4}{3} (\vec{S}_1 \cdot \vec{v}_2)^2 + \frac{8}{3} (\hat{n} \cdot \vec{v}_2)^2 \vec{S}_1 \cdot \vec{S}_1 + \frac{8}{3} \hat{n} \cdot \vec{S}_1 \hat{n} \cdot \vec{v}_1 \vec{S}_1 \cdot \vec{a}_2 + \frac{8}{3} \hat{n} \cdot \vec{S}_1 \hat{n} \cdot \vec{v}_2 \vec{S}_1 \cdot \vec{a}_2 + \\
& \frac{8}{3} \hat{n} \cdot \vec{a}_2 \hat{n} \cdot \vec{S}_1 \vec{S}_1 \cdot \vec{v}_1 + \frac{8}{3} \hat{n} \cdot \vec{a}_2 \hat{n} \cdot \vec{S}_1 \vec{S}_1 \cdot \vec{v}_2 - \frac{8}{3} \hat{n} \cdot \vec{S}_1 \hat{n} \cdot \vec{v}_2 \vec{S}_1 \cdot \vec{v}_2 + \frac{2}{3} (\hat{n} \cdot \vec{S}_1)^2 \vec{a}_1 \cdot \vec{a}_2 - \\
& \frac{16}{3} \hat{n} \cdot \vec{a}_2 \hat{n} \cdot \vec{v}_1 \vec{S}_1 \cdot \vec{S}_1 - \frac{16}{3} \hat{n} \cdot \vec{a}_2 \hat{n} \cdot \vec{v}_2 \vec{S}_1 \cdot \vec{S}_1 + \frac{8}{3} (\hat{n} \cdot \vec{v}_2)^2 \vec{S}_1 \cdot \vec{S}_1 + \frac{4}{3} \hat{n} \cdot \vec{a}_2 \hat{n} \cdot \vec{S}_1 \vec{S}_1 \cdot \vec{a}_1 + \\
& \frac{4}{3} \hat{n} \cdot \vec{a}_1 \hat{n} \cdot \vec{S}_1 \vec{S}_1 \cdot \vec{a}_2 - \frac{4}{3} \vec{S}_1 \cdot \vec{v}_1 \vec{S}_1 \cdot \vec{a}_2 - \frac{4}{3} \vec{S}_1 \cdot \vec{v}_2 \vec{S}_1 \cdot \vec{a}_2 - \frac{2}{3} \vec{S}_1 \cdot \vec{a}_1 \vec{S}_1 \cdot \vec{a}_2 - \frac{4}{3} \hat{n} \cdot \vec{a}_1 \hat{n} \cdot \vec{a}_2 \vec{S}_1 \cdot \vec{S}_1 + \\
& \frac{2}{3} \vec{a}_1 \cdot \vec{a}_2 \vec{S}_1 \cdot \vec{S}_1 - \frac{4}{3} \vec{S}_1 \cdot \vec{a}_2 \vec{S}_1 \cdot \vec{v}_1 - \frac{8}{3} \hat{n} \cdot \vec{S}_1 \hat{n} \cdot \vec{v}_2 \vec{S}_1 \cdot \vec{v}_2 - \frac{4}{3} \vec{S}_1 \cdot \vec{a}_2 \vec{S}_1 \cdot \vec{v}_2 + \frac{4}{3} \vec{S}_1 \cdot \vec{v}_2 \vec{S}_1 \cdot \vec{v}_2 + \\
& \left. \frac{8}{3} \vec{S}_1 \cdot \vec{S}_1 \vec{v}_1 \cdot \vec{a}_2 + \frac{8}{3} \vec{S}_1 \cdot \vec{S}_1 \vec{v}_2 \cdot \vec{a}_2 - \frac{4}{3} \hat{n} \cdot \vec{S}_1 \hat{n} \cdot \vec{S}_1 \vec{v}_2 \cdot \vec{v}_2 - \frac{4}{3} \vec{S}_1 \cdot \vec{S}_1 \vec{v}_2 \cdot \vec{v}_2 - \frac{4}{3} \vec{S}_1 \cdot \vec{S}_1 \vec{v}_2 \cdot \vec{v}_2 \right) + \frac{1}{r^3} \\
& \left( -32 \hat{n} \cdot \vec{S}_1 \hat{n} \cdot \vec{S}_1 (\hat{n} \cdot \vec{v}_2)^3 - \frac{32}{3} \vec{S}_1 \cdot \vec{S}_1 (\hat{n} \cdot \vec{v}_2)^3 - 16 \hat{n} \cdot \vec{a}_1 (\hat{n} \cdot \vec{S}_1)^2 (\hat{n} \cdot \vec{v}_2)^2 - 64 \hat{n} \cdot \vec{S}_1 \hat{n} \cdot \vec{S}_1 \hat{n} \cdot \vec{v}_1 (\hat{n} \cdot \vec{v}_2)^2 + \right. \\
& \left. \frac{32}{3} \hat{n} \cdot \vec{S}_1 \vec{S}_1 \cdot \vec{v}_1 (\hat{n} \cdot \vec{v}_2)^2 + 16 \hat{n} \cdot \vec{S}_1 \vec{S}_1 \cdot \vec{v}_2 (\hat{n} \cdot \vec{v}_2)^2 - \frac{64}{3} \hat{n} \cdot \vec{v}_1 \vec{S}_1 \cdot \vec{S}_1 (\hat{n} \cdot \vec{v}_2)^2 + \frac{16}{3} \hat{n} \cdot \vec{S}_1 \vec{S}_1 \cdot \vec{a}_1 (\hat{n} \cdot \vec{v}_2)^2 - \right.
\end{aligned}$$



$$\{\text{DiagS1CES2}[2, 2, 40],$$

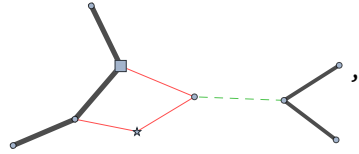

[illegible]

$$\begin{aligned}
& \frac{5}{6} \hat{n} \cdot \vec{v}_2 \vec{S}_1 \cdot \vec{v}_2 \vec{S}_1 \cdot \vec{v}_1 + \frac{1}{3} \hat{n} \cdot \vec{v}_2 \vec{S}_1 \cdot \vec{a}_1 \vec{S}_1 \cdot \vec{v}_1 + \frac{1}{6} \hat{n} \cdot \vec{v}_1 \vec{S}_1 \cdot \vec{a}_2 \vec{S}_1 \cdot \vec{v}_1 - \frac{1}{4} \hat{n} \cdot \vec{S}_1 (\hat{n} \cdot \vec{v}_1)^2 \vec{S}_1 \cdot \vec{v}_2 + \\
& \frac{1}{3} \hat{n} \cdot \vec{S}_1 \hat{n} \cdot \vec{v}_1 \hat{n} \cdot \vec{v}_2 \vec{S}_1 \cdot \vec{v}_2 + \frac{1}{2} \hat{n} \cdot \vec{v}_1 \vec{S}_1 \cdot \vec{v}_1 \vec{S}_1 \cdot \vec{v}_2 - \frac{5}{6} \hat{n} \cdot \vec{v}_2 \vec{S}_1 \cdot \vec{v}_1 \vec{S}_1 \cdot \vec{v}_2 - \frac{1}{3} \hat{n} \cdot \vec{v}_1 \vec{S}_1 \cdot \vec{v}_2 \vec{S}_1 \cdot \vec{v}_2 + \\
& \frac{1}{3} \hat{n} \cdot \vec{v}_1 \vec{S}_1 \cdot \vec{a}_1 \vec{S}_1 \cdot \vec{v}_2 - \frac{7}{6} \hat{n} \cdot \vec{v}_2 \vec{S}_1 \cdot \vec{a}_1 \vec{S}_1 \cdot \vec{v}_2 - \frac{1}{6} \hat{n} \cdot \vec{a}_1 \vec{S}_1 \cdot \vec{v}_1 \vec{S}_1 \cdot \vec{v}_2 + \frac{1}{6} \hat{n} \cdot \vec{v}_2 \vec{S}_1 \cdot \vec{S}_1 \vec{v}_1 \cdot \vec{a}_1 - \\
& \frac{2}{3} \hat{n} \cdot \vec{v}_1 \vec{S}_1 \cdot \vec{S}_1 \vec{v}_1 \cdot \vec{a}_2 - \frac{5}{4} \hat{n} \cdot \vec{v}_2 \vec{S}_1 \cdot \vec{S}_1 \vec{v}_1 \cdot \vec{v}_1 - \frac{7}{12} \hat{n} \cdot \vec{a}_2 \vec{S}_1 \cdot \vec{S}_1 \vec{v}_1 \cdot \vec{v}_1 - \frac{1}{4} \hat{n} \cdot \vec{S}_1 \vec{S}_1 \cdot \vec{v}_2 \vec{v}_1 \cdot \vec{v}_1 - \\
& \frac{5}{2} \hat{n} \cdot \vec{v}_1 \vec{S}_1 \cdot \vec{S}_1 \vec{v}_1 \cdot \vec{v}_2 + \frac{5}{3} \hat{n} \cdot \vec{v}_2 \vec{S}_1 \cdot \vec{S}_1 \vec{v}_1 \cdot \vec{v}_2 - \frac{5}{6} \hat{n} \cdot \vec{a}_1 \vec{S}_1 \cdot \vec{S}_1 \vec{v}_1 \cdot \vec{v}_2 - \frac{1}{2} \hat{n} \cdot \vec{S}_1 \vec{S}_1 \cdot \vec{v}_1 \vec{v}_1 \cdot \vec{v}_2 + \\
& \frac{7}{6} \hat{n} \cdot \vec{S}_1 \vec{S}_1 \cdot \vec{v}_2 \vec{v}_1 \cdot \vec{v}_2 + \frac{1}{3} \hat{n} \cdot \vec{v}_1 \vec{S}_1 \cdot \vec{S}_1 \vec{v}_2 \cdot \vec{v}_2 + \frac{1}{3} \hat{n} \cdot \vec{a}_1 \vec{S}_1 \cdot \vec{S}_1 \vec{v}_2 \cdot \vec{v}_2 - \frac{1}{6} \hat{n} \cdot \vec{S}_1 \vec{S}_1 \cdot \vec{v}_1 \vec{v}_2 \cdot \vec{v}_2 \Big) + \frac{1}{r^4} \\
& \left\{ 7 (\hat{n} \cdot \vec{S}_1)^2 \hat{n} \cdot \vec{v}_2 (\hat{n} \cdot \vec{v}_1)^3 - 2 \hat{n} \cdot \vec{v}_2 \vec{S}_1 \cdot \vec{S}_1 (\hat{n} \cdot \vec{v}_1)^3 - \frac{1}{4} \hat{n} \cdot \vec{S}_1 \vec{S}_1 \cdot \vec{v}_2 (\hat{n} \cdot \vec{v}_1)^3 - 10 (\hat{n} \cdot \vec{S}_1)^2 (\hat{n} \cdot \vec{v}_2)^2 (\hat{n} \cdot \vec{v}_1)^2 - \right. \\
& \frac{1}{6} (\vec{S}_1 \cdot \vec{v}_2)^2 (\hat{n} \cdot \vec{v}_1)^2 + \frac{7}{2} (\hat{n} \cdot \vec{v}_2)^2 \vec{S}_1 \cdot \vec{S}_1 (\hat{n} \cdot \vec{v}_1)^2 - \frac{3}{4} \hat{n} \cdot \vec{S}_1 \hat{n} \cdot \vec{v}_2 \vec{S}_1 \cdot \vec{v}_1 (\hat{n} \cdot \vec{v}_1)^2 + \\
& \frac{7}{2} \hat{n} \cdot \vec{S}_1 \hat{n} \cdot \vec{v}_2 \vec{S}_1 \cdot \vec{v}_2 (\hat{n} \cdot \vec{v}_1)^2 - \frac{1}{2} \vec{S}_1 \cdot \vec{v}_1 \vec{S}_1 \cdot \vec{v}_2 (\hat{n} \cdot \vec{v}_1)^2 - \frac{39}{4} (\hat{n} \cdot \vec{S}_1)^2 \vec{v}_1 \cdot \vec{v}_2 (\hat{n} \cdot \vec{v}_1)^2 + \\
& \frac{9}{4} \vec{S}_1 \cdot \vec{S}_1 \vec{v}_1 \cdot \vec{v}_2 (\hat{n} \cdot \vec{v}_1)^2 + \frac{5}{4} (\hat{n} \cdot \vec{S}_1)^2 \vec{v}_2 \cdot \vec{v}_2 (\hat{n} \cdot \vec{v}_1)^2 - \frac{7}{12} \vec{S}_1 \cdot \vec{S}_1 \vec{v}_2 \cdot \vec{v}_2 (\hat{n} \cdot \vec{v}_1)^2 - \frac{1}{2} \hat{n} \cdot \vec{v}_2 (\vec{S}_1 \cdot \vec{v}_1)^2 \hat{n} \cdot \vec{v}_1 - \\
& 4 \hat{n} \cdot \vec{S}_1 (\hat{n} \cdot \vec{v}_2)^2 \vec{S}_1 \cdot \vec{v}_1 \hat{n} \cdot \vec{v}_1 + \frac{4}{3} \hat{n} \cdot \vec{v}_2 \vec{S}_1 \cdot \vec{v}_1 \vec{S}_1 \cdot \vec{v}_2 \hat{n} \cdot \vec{v}_1 - \frac{39}{4} (\hat{n} \cdot \vec{S}_1)^2 \hat{n} \cdot \vec{v}_2 \vec{v}_1 \cdot \vec{v}_1 \hat{n} \cdot \vec{v}_1 + \\
& \frac{9}{4} \hat{n} \cdot \vec{v}_2 \vec{S}_1 \cdot \vec{S}_1 \vec{v}_1 \cdot \vec{v}_1 \hat{n} \cdot \vec{v}_1 + \frac{7}{4} \hat{n} \cdot \vec{S}_1 \vec{S}_1 \cdot \vec{v}_2 \vec{v}_1 \cdot \vec{v}_1 \hat{n} \cdot \vec{v}_1 + \frac{25}{2} (\hat{n} \cdot \vec{S}_1)^2 \hat{n} \cdot \vec{v}_2 \vec{v}_1 \cdot \vec{v}_2 \hat{n} \cdot \vec{v}_1 - \\
& \frac{23}{6} \hat{n} \cdot \vec{v}_2 \vec{S}_1 \cdot \vec{S}_1 \vec{v}_1 \cdot \vec{v}_2 \hat{n} \cdot \vec{v}_1 + \frac{7}{2} \hat{n} \cdot \vec{S}_1 \vec{S}_1 \cdot \vec{v}_1 \vec{v}_1 \cdot \vec{v}_2 \hat{n} \cdot \vec{v}_1 - \frac{11}{3} \hat{n} \cdot \vec{S}_1 \vec{S}_1 \cdot \vec{v}_2 \vec{v}_1 \cdot \vec{v}_2 \hat{n} \cdot \vec{v}_1 + \\
& \frac{2}{3} \hat{n} \cdot \vec{S}_1 \vec{S}_1 \cdot \vec{v}_1 \vec{v}_2 \cdot \vec{v}_2 \hat{n} \cdot \vec{v}_1 + \frac{4}{3} (\hat{n} \cdot \vec{v}_2)^2 (\vec{S}_1 \cdot \vec{v}_1)^2 - \frac{5}{3} (\hat{n} \cdot \vec{S}_1)^2 (\vec{v}_1 \cdot \vec{v}_2)^2 + \frac{2}{3} \vec{S}_1 \cdot \vec{S}_1 (\vec{v}_1 \cdot \vec{v}_2)^2 + \\
& \frac{25}{2} (\hat{n} \cdot \vec{S}_1)^2 (\hat{n} \cdot \vec{v}_2)^2 \vec{v}_1 \cdot \vec{v}_1 + \frac{2}{3} (\vec{S}_1 \cdot \vec{v}_2)^2 \vec{v}_1 \cdot \vec{v}_1 - \frac{7}{3} (\hat{n} \cdot \vec{v}_2)^2 \vec{S}_1 \cdot \vec{S}_1 \vec{v}_1 \cdot \vec{v}_1 + \frac{7}{4} \hat{n} \cdot \vec{S}_1 \hat{n} \cdot \vec{v}_2 \vec{S}_1 \cdot \vec{v}_1 \vec{v}_1 \cdot \vec{v}_1 - \\
& \frac{41}{6} \hat{n} \cdot \vec{S}_1 \hat{n} \cdot \vec{v}_2 \vec{S}_1 \cdot \vec{v}_2 \vec{v}_1 \cdot \vec{v}_1 + \frac{4}{3} \hat{n} \cdot \vec{S}_1 \hat{n} \cdot \vec{v}_2 \vec{S}_1 \cdot \vec{v}_1 \vec{v}_1 \cdot \vec{v}_2 - \frac{1}{3} \vec{S}_1 \cdot \vec{v}_1 \vec{S}_1 \cdot \vec{v}_2 \vec{v}_1 \cdot \vec{v}_2 + \frac{3}{2} (\hat{n} \cdot \vec{S}_1)^2 \vec{v}_1 \cdot \vec{v}_1 \vec{v}_1 \cdot \vec{v}_2 - \\
& \left. \frac{1}{2} \vec{S}_1 \cdot \vec{S}_1 \vec{v}_1 \cdot \vec{v}_1 \vec{v}_1 \cdot \vec{v}_2 - \frac{1}{3} (\vec{S}_1 \cdot \vec{v}_1)^2 \vec{v}_2 \cdot \vec{v}_2 - \frac{25}{12} (\hat{n} \cdot \vec{S}_1)^2 \vec{v}_1 \cdot \vec{v}_1 \vec{v}_2 \cdot \vec{v}_2 + \frac{7}{12} \vec{S}_1 \cdot \vec{S}_1 \vec{v}_1 \cdot \vec{v}_1 \vec{v}_2 \cdot \vec{v}_2 \right) \Big\} m_2 C_{ES^2 1} \Big\}
\end{aligned}$$

{DiagS1CES2[2, 2, 41],

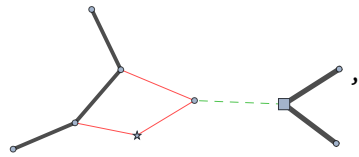

$$\begin{aligned}
& \frac{1}{m_1} G^2 \left( \frac{1}{r} \left( -\frac{2}{3} \hat{n} \cdot \vec{a}_2 \left( \hat{n} \cdot \vec{S}_1 \right)^2 - \frac{1}{3} \vec{S}_1 \cdot \vec{a}_2 \hat{n} \cdot \vec{S}_1 - \frac{2}{3} \hat{n} \cdot \vec{S}_1 \hat{n} \cdot \vec{a}_2 \hat{n} \cdot \vec{S}_1 + \right. \right. \\
& \left. \frac{1}{3} \hat{n} \cdot \vec{a}_2 \vec{S}_1 \cdot \vec{S}_1 - \frac{1}{6} \hat{n} \cdot \vec{S}_1 \vec{S}_1 \cdot \vec{a}_2 + \frac{1}{3} \hat{n} \cdot \vec{a}_2 \vec{S}_1 \cdot \vec{S}_1 - \frac{1}{6} \hat{n} \cdot \vec{S}_1 \vec{S}_1 \cdot \vec{a}_2 \right) + \frac{1}{r^2} \\
& \left( -\frac{4}{3} (\hat{n} \cdot \vec{v}_2)^2 \left( \hat{n} \cdot \vec{S}_1 \right)^2 + \frac{4}{3} \vec{v}_2 \cdot \vec{v}_2 \left( \hat{n} \cdot \vec{S}_1 \right)^2 + \frac{16}{3} \hat{n} \cdot \vec{a}_2 \hat{n} \cdot \vec{S}_1 \hat{n} \cdot \vec{v}_1 \hat{n} \cdot \vec{S}_1 - \frac{8}{3} \hat{n} \cdot \vec{a}_2 \hat{n} \cdot \vec{S}_1 \hat{n} \cdot \vec{v}_2 \hat{n} \cdot \vec{S}_1 + \right. \\
& \frac{4}{3} \hat{n} \cdot \vec{v}_2 \vec{S}_1 \cdot \vec{v}_2 \hat{n} \cdot \vec{S}_1 - \frac{1}{3} \hat{n} \cdot \vec{v}_1 \vec{S}_1 \cdot \vec{a}_2 \hat{n} \cdot \vec{S}_1 - \frac{1}{3} \hat{n} \cdot \vec{v}_2 \vec{S}_1 \cdot \vec{a}_2 \hat{n} \cdot \vec{S}_1 - \frac{4}{3} \hat{n} \cdot \vec{a}_2 \vec{S}_1 \cdot \vec{v}_1 \hat{n} \cdot \vec{S}_1 + \frac{5}{3} \hat{n} \cdot \vec{a}_2 \vec{S}_1 \cdot \vec{v}_2 \hat{n} \cdot \vec{S}_1 + \\
& \frac{2}{3} \hat{n} \cdot \vec{S}_1 \vec{v}_1 \cdot \vec{a}_2 \hat{n} \cdot \vec{S}_1 - \frac{4}{3} \hat{n} \cdot \vec{S}_1 \vec{v}_2 \cdot \vec{a}_2 \hat{n} \cdot \vec{S}_1 + \frac{4}{3} \hat{n} \cdot \vec{a}_1 \hat{n} \cdot \vec{a}_2 \left( \hat{n} \cdot \vec{S}_1 \right)^2 - \frac{4}{3} \hat{n} \cdot \vec{S}_1 \hat{n} \cdot \vec{S}_1 (\hat{n} \cdot \vec{v}_2)^2 - \frac{1}{3} \left( \frac{1}{\vec{S}_1 \cdot \vec{v}_2} \right)^2 - \\
& \left. \frac{2}{3} (\hat{n} \cdot \vec{v}_2)^2 \frac{1}{\vec{S}_1 \cdot \vec{S}_1} - \frac{1}{3} \hat{n} \cdot \vec{S}_1 \hat{n} \cdot \vec{v}_1 \vec{S}_1 \cdot \vec{a}_2 - \frac{1}{3} \hat{n} \cdot \vec{S}_1 \hat{n} \cdot \vec{v}_2 \vec{S}_1 \cdot \vec{a}_2 - \frac{4}{3} \hat{n} \cdot \vec{a}_2 \hat{n} \cdot \vec{S}_1 \vec{S}_1 \cdot \vec{v}_1 + \frac{5}{3} \hat{n} \cdot \vec{a}_2 \hat{n} \cdot \vec{S}_1 \vec{S}_1 \cdot \vec{v}_2 + \right.
\end{aligned}$$



$$\begin{aligned} & \frac{16}{3} \hat{n} \cdot \vec{v}_1 \vec{S}_1 \cdot \vec{S}_1 \vec{v}_1 \cdot \vec{v}_2 \hat{n} \cdot \vec{v}_2 - \frac{16}{3} \hat{n} \cdot \vec{S}_1 \vec{S}_1 \cdot \vec{v}_1 \vec{v}_1 \cdot \vec{v}_2 \hat{n} \cdot \vec{v}_2 + 8 \hat{n} \cdot \vec{S}_1 \vec{S}_1 \cdot \vec{v}_2 \vec{v}_1 \cdot \vec{v}_2 \hat{n} \cdot \vec{v}_2 - \\ & 12 \left( \hat{n} \cdot \vec{S}_1 \right)^2 \hat{n} \cdot \vec{v}_1 \vec{v}_2 \cdot \vec{v}_2 \hat{n} \cdot \vec{v}_2 - 2 \hat{n} \cdot \vec{v}_1 \vec{S}_1 \cdot \vec{S}_1 \vec{v}_2 \cdot \vec{v}_2 \hat{n} \cdot \vec{v}_2 + 4 \hat{n} \cdot \vec{S}_1 \vec{S}_1 \cdot \vec{v}_1 \vec{v}_2 \cdot \vec{v}_2 \hat{n} \cdot \vec{v}_2 - \\ & \frac{4}{3} \left( \hat{n} \cdot \vec{v}_1 \right)^2 \left( \vec{S}_1 \cdot \vec{v}_2 \right)^2 - \frac{4}{3} \left( \hat{n} \cdot \vec{S}_1 \right)^2 \left( \vec{v}_1 \cdot \vec{v}_2 \right)^2 - \frac{2}{3} \vec{S}_1 \cdot \vec{S}_1 \left( \vec{v}_1 \cdot \vec{v}_2 \right)^2 + \frac{1}{3} \left( \vec{S}_1 \cdot \vec{v}_2 \right)^2 \vec{v}_1 \cdot \vec{v}_1 - \\ & \left( \vec{S}_1 \cdot \vec{v}_2 \right)^2 \vec{v}_1 \cdot \vec{v}_2 - \frac{16}{3} \hat{n} \cdot \vec{S}_1 \hat{n} \cdot \vec{v}_1 \vec{S}_1 \cdot \vec{v}_2 \vec{v}_1 \cdot \vec{v}_2 + \frac{4}{3} \vec{S}_1 \cdot \vec{v}_1 \vec{S}_1 \cdot \vec{v}_2 \vec{v}_1 \cdot \vec{v}_2 + 16 \left( \hat{n} \cdot \vec{S}_1 \right)^2 \left( \hat{n} \cdot \vec{v}_1 \right)^2 \vec{v}_2 \cdot \vec{v}_2 + \\ & \frac{4}{3} \left( \vec{S}_1 \cdot \vec{v}_1 \right)^2 \vec{v}_2 \cdot \vec{v}_2 + \frac{4}{3} \left( \hat{n} \cdot \vec{v}_1 \right)^2 \vec{S}_1 \cdot \vec{S}_1 \vec{v}_2 \cdot \vec{v}_2 - \frac{32}{3} \hat{n} \cdot \vec{S}_1 \hat{n} \cdot \vec{v}_1 \vec{S}_1 \cdot \vec{v}_1 \vec{v}_2 \cdot \vec{v}_2 + 4 \hat{n} \cdot \vec{S}_1 \hat{n} \cdot \vec{v}_1 \vec{S}_1 \cdot \vec{v}_2 \vec{v}_2 \cdot \vec{v}_2 - \\ & \vec{S}_1 \cdot \vec{v}_1 \vec{S}_1 \cdot \vec{v}_2 \vec{v}_2 \cdot \vec{v}_2 - \frac{8}{3} \left( \hat{n} \cdot \vec{S}_1 \right)^2 \vec{v}_1 \cdot \vec{v}_1 \vec{v}_2 \cdot \vec{v}_2 - \frac{1}{3} \vec{S}_1 \cdot \vec{S}_1 \vec{v}_1 \cdot \vec{v}_1 \vec{v}_2 \cdot \vec{v}_2 + 2 \vec{S}_1 \cdot \vec{S}_1 \vec{v}_1 \cdot \vec{v}_2 \vec{v}_2 \cdot \vec{v}_2 \Big) \Big) m_2^2 C_{\text{ES}^2_1} \} \end{aligned}$$

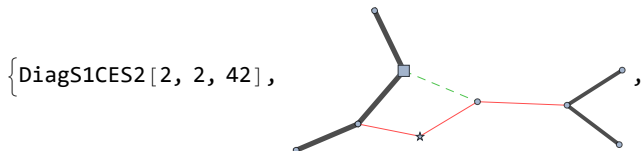

[illegible]





$$\begin{aligned}
& \frac{8}{3} \hat{n} \cdot \vec{v}_2 \vec{S}_1 \cdot \vec{S}_1 \vec{v}_1 \cdot \vec{v}_2 \hat{n} \cdot \vec{v}_1 - \frac{3}{2} \hat{n} \cdot \vec{S}_1 \vec{S}_1 \cdot \vec{v}_1 \vec{v}_1 \cdot \vec{v}_2 \hat{n} \cdot \vec{v}_1 + \frac{4}{3} \hat{n} \cdot \vec{S}_1 \vec{S}_1 \cdot \vec{v}_2 \vec{v}_1 \cdot \vec{v}_2 \hat{n} \cdot \vec{v}_1 - \\
& \frac{4}{3} \hat{n} \cdot \vec{S}_1 \vec{S}_1 \cdot \vec{v}_1 \vec{v}_2 \cdot \vec{v}_2 \hat{n} \cdot \vec{v}_1 - \frac{8}{3} (\hat{n} \cdot \vec{v}_2)^2 (\vec{S}_1 \cdot \vec{v}_1)^2 - \frac{15}{8} (\hat{n} \cdot \vec{S}_1)^2 (\vec{v}_1 \cdot \vec{v}_1)^2 + \frac{5}{8} \vec{S}_1 \cdot \vec{S}_1 (\vec{v}_1 \cdot \vec{v}_1)^2 + \\
& \frac{1}{3} (\hat{n} \cdot \vec{S}_1)^2 (\vec{v}_1 \cdot \vec{v}_2)^2 - \frac{1}{3} \vec{S}_1 \cdot \vec{S}_1 (\vec{v}_1 \cdot \vec{v}_2)^2 - 16 (\hat{n} \cdot \vec{S}_1)^2 (\hat{n} \cdot \vec{v}_2)^2 \vec{v}_1 \cdot \vec{v}_1 - \frac{4}{3} (\vec{S}_1 \cdot \vec{v}_2)^2 \vec{v}_1 \cdot \vec{v}_1 + \\
& \frac{8}{3} (\hat{n} \cdot \vec{v}_2)^2 \vec{S}_1 \cdot \vec{S}_1 \vec{v}_1 \cdot \vec{v}_1 + 3 \hat{n} \cdot \vec{S}_1 \hat{n} \cdot \vec{v}_2 \vec{S}_1 \cdot \vec{v}_1 \vec{v}_1 \cdot \vec{v}_1 + \frac{32}{3} \hat{n} \cdot \vec{S}_1 \hat{n} \cdot \vec{v}_2 \vec{S}_1 \cdot \vec{v}_2 \vec{v}_1 \cdot \vec{v}_1 - \frac{3}{4} \vec{S}_1 \cdot \vec{v}_1 \vec{S}_1 \cdot \vec{v}_2 \vec{v}_1 \cdot \vec{v}_1 + \\
& \frac{3}{4} (\vec{S}_1 \cdot \vec{v}_1)^2 \vec{v}_1 \cdot \vec{v}_2 - \frac{8}{3} \hat{n} \cdot \vec{S}_1 \hat{n} \cdot \vec{v}_2 \vec{S}_1 \cdot \vec{v}_1 \vec{v}_1 \cdot \vec{v}_2 + \frac{2}{3} \vec{S}_1 \cdot \vec{v}_1 \vec{S}_1 \cdot \vec{v}_2 \vec{v}_1 \cdot \vec{v}_2 + \frac{9}{8} (\hat{n} \cdot \vec{S}_1)^2 \vec{v}_1 \cdot \vec{v}_1 \vec{v}_1 \cdot \vec{v}_2 - \\
& \frac{3}{8} \vec{S}_1 \cdot \vec{S}_1 \vec{v}_1 \cdot \vec{v}_1 \vec{v}_1 \cdot \vec{v}_2 + \frac{2}{3} (\vec{S}_1 \cdot \vec{v}_1)^2 \vec{v}_2 \cdot \vec{v}_2 + \frac{8}{3} (\hat{n} \cdot \vec{S}_1)^2 \vec{v}_1 \cdot \vec{v}_1 \vec{v}_2 \cdot \vec{v}_2 - \frac{2}{3} \vec{S}_1 \cdot \vec{S}_1 \vec{v}_1 \cdot \vec{v}_1 \vec{v}_2 \cdot \vec{v}_2 \Big) \Big) m_2 C_{ES^2_1} \}
\end{aligned}$$

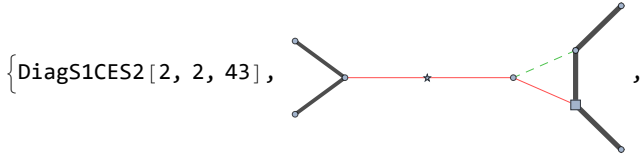

$$\begin{aligned}
& G^2 \left( \frac{1}{\rho^2} \left( 4 \hat{n} \cdot \vec{v}_1 \hat{n} \cdot \vec{v}_2 \left( \hat{n} \cdot \vec{S}_1 \right)^2 - \vec{v}_1 \cdot \vec{v}_2 \left( \hat{n} \cdot \vec{S}_1 \right)^2 - \frac{10}{3} \hat{n} \cdot \vec{a}_2 \hat{n} \cdot \vec{S}_1 \hat{n} \cdot \vec{v}_1 \hat{n} \cdot \vec{S}_1 + 4 \hat{n} \cdot \vec{a}_1 \hat{n} \cdot \vec{S}_1 \hat{n} \cdot \vec{v}_2 \hat{n} \cdot \vec{S}_1 - \right. \right. \\
& 2 \hat{n} \cdot \vec{v}_2 \vec{S}_1 \cdot \vec{v}_1 \hat{n} \cdot \vec{S}_1 - 2 \hat{n} \cdot \vec{v}_1 \vec{S}_1 \cdot \vec{v}_2 \hat{n} \cdot \vec{S}_1 - \hat{n} \cdot \vec{S}_1 \vec{a}_1 \cdot \vec{v}_2 \hat{n} \cdot \vec{S}_1 - \hat{n} \cdot \vec{v}_2 \vec{S}_1 \cdot \vec{a}_1 \hat{n} \cdot \vec{S}_1 + \frac{5}{6} \hat{n} \cdot \vec{v}_1 \vec{S}_1 \cdot \vec{a}_2 \hat{n} \cdot \vec{S}_1 + \\
& \frac{1}{3} \hat{n} \cdot \vec{a}_2 \vec{S}_1 \cdot \vec{v}_1 \hat{n} \cdot \vec{S}_1 - \hat{n} \cdot \vec{a}_1 \vec{S}_1 \cdot \vec{v}_2 \hat{n} \cdot \vec{S}_1 + \frac{5}{6} \hat{n} \cdot \vec{S}_1 \vec{v}_1 \cdot \vec{a}_2 \hat{n} \cdot \vec{S}_1 - \frac{5}{3} \hat{n} \cdot \vec{a}_1 \hat{n} \cdot \vec{a}_2 (\hat{n} \cdot \vec{S}_1)^2 + \\
& 4 \hat{n} \cdot \vec{S}_1 \hat{n} \cdot \vec{S}_1 \hat{n} \cdot \vec{v}_1 \hat{n} \cdot \vec{v}_2 - \hat{n} \cdot \vec{S}_1 \hat{n} \cdot \vec{v}_2 \vec{S}_1 \cdot \vec{a}_1 + \frac{5}{6} \hat{n} \cdot \vec{S}_1 \hat{n} \cdot \vec{v}_1 \vec{S}_1 \cdot \vec{a}_2 + \frac{1}{3} \hat{n} \cdot \vec{a}_2 \hat{n} \cdot \vec{S}_1 \vec{S}_1 \cdot \vec{v}_1 - \hat{n} \cdot \vec{a}_1 \hat{n} \cdot \vec{S}_1 \vec{S}_1 \cdot \vec{v}_2 + \\
& \frac{1}{S_1 \cdot \vec{v}_1} \vec{S}_1 \cdot \vec{v}_2 - \hat{n} \cdot \vec{S}_1 \hat{n} \cdot \vec{v}_2 \vec{S}_1 \cdot \vec{v}_1 - \hat{n} \cdot \vec{S}_1 \hat{n} \cdot \vec{v}_1 \vec{S}_1 \cdot \vec{v}_2 + \frac{5}{12} (\hat{n} \cdot \vec{S}_1)^2 \vec{a}_1 \cdot \vec{a}_2 + \frac{1}{3} \hat{n} \cdot \vec{a}_2 \hat{n} \cdot \vec{v}_1 \vec{S}_1 \cdot \vec{S}_1 + \\
& \frac{1}{3} \hat{n} \cdot \vec{a}_2 \hat{n} \cdot \vec{S}_1 \vec{S}_1 \cdot \vec{a}_1 + \frac{1}{2} \vec{S}_1 \cdot \vec{v}_2 \vec{S}_1 \cdot \vec{a}_1 + \frac{5}{6} \hat{n} \cdot \vec{a}_1 \hat{n} \cdot \vec{S}_1 \vec{S}_1 \cdot \vec{a}_2 - \frac{1}{6} \vec{S}_1 \cdot \vec{v}_1 \vec{S}_1 \cdot \vec{a}_2 - \frac{1}{6} \vec{S}_1 \cdot \vec{a}_1 \vec{S}_1 \cdot \vec{a}_2 + \\
& \frac{1}{6} \hat{n} \cdot \vec{a}_1 \hat{n} \cdot \vec{a}_2 \vec{S}_1 \cdot \vec{S}_1 - \frac{1}{12} \vec{a}_1 \cdot \vec{a}_2 \vec{S}_1 \cdot \vec{S}_1 - \hat{n} \cdot \vec{S}_1 \hat{n} \cdot \vec{v}_2 \vec{S}_1 \cdot \vec{v}_1 - \frac{1}{6} \vec{S}_1 \cdot \vec{a}_2 \vec{S}_1 \cdot \vec{v}_1 + \frac{1}{2} \vec{S}_1 \cdot \vec{v}_2 \vec{S}_1 \cdot \vec{v}_1 - \\
& \hat{n} \cdot \vec{S}_1 \hat{n} \cdot \vec{v}_1 \vec{S}_1 \cdot \vec{v}_2 + \frac{1}{2} \vec{S}_1 \cdot \vec{a}_1 \vec{S}_1 \cdot \vec{v}_2 + \frac{1}{2} \vec{S}_1 \cdot \vec{v}_1 \vec{S}_1 \cdot \vec{v}_2 - \frac{1}{6} \vec{S}_1 \cdot \vec{S}_1 \vec{v}_1 \cdot \vec{a}_2 - \hat{n} \cdot \vec{S}_1 \hat{n} \cdot \vec{S}_1 \vec{v}_1 \cdot \vec{v}_2 \Big) + \\
& \frac{1}{\rho^3} \left( 10 \hat{n} \cdot \vec{a}_2 (\hat{n} \cdot \vec{v}_1)^2 (\hat{n} \cdot \vec{S}_1)^2 - 10 \hat{n} \cdot \vec{a}_1 (\hat{n} \cdot \vec{v}_2)^2 (\hat{n} \cdot \vec{S}_1)^2 - 20 \hat{n} \cdot \vec{a}_1 \hat{n} \cdot \vec{v}_1 \hat{n} \cdot \vec{v}_2 (\hat{n} \cdot \vec{S}_1)^2 + \right. \\
& \frac{10}{3} \hat{n} \cdot \vec{v}_1 \vec{a}_1 \cdot \vec{v}_2 (\hat{n} \cdot \vec{S}_1)^2 + \frac{10}{3} \hat{n} \cdot \vec{v}_2 \vec{a}_1 \cdot \vec{v}_2 (\hat{n} \cdot \vec{S}_1)^2 + \frac{10}{3} \hat{n} \cdot \vec{v}_2 \vec{v}_1 \cdot \vec{a}_1 (\hat{n} \cdot \vec{S}_1)^2 - \\
& \frac{10}{3} \hat{n} \cdot \vec{v}_1 \vec{v}_1 \cdot \vec{a}_2 (\hat{n} \cdot \vec{S}_1)^2 - \frac{5}{3} \hat{n} \cdot \vec{a}_2 \vec{v}_1 \cdot \vec{v}_1 (\hat{n} \cdot \vec{S}_1)^2 + \frac{10}{3} \hat{n} \cdot \vec{a}_1 \vec{v}_1 \cdot \vec{v}_2 (\hat{n} \cdot \vec{S}_1)^2 + \frac{5}{3} \hat{n} \cdot \vec{a}_1 \vec{v}_2 \cdot \vec{v}_2 (\hat{n} \cdot \vec{S}_1)^2 - \\
& 20 \hat{n} \cdot \vec{S}_1 \hat{n} \cdot \vec{v}_1 (\hat{n} \cdot \vec{v}_2)^2 \hat{n} \cdot \vec{S}_1 - 44 \hat{n} \cdot \vec{S}_1 (\hat{n} \cdot \vec{v}_1)^2 \hat{n} \cdot \vec{v}_2 \hat{n} \cdot \vec{S}_1 + \frac{4}{3} (\hat{n} \cdot \vec{v}_2)^2 \vec{S}_1 \cdot \vec{v}_1 \hat{n} \cdot \vec{S}_1 + \\
& \frac{38}{3} \hat{n} \cdot \vec{v}_1 \hat{n} \cdot \vec{v}_2 \vec{S}_1 \cdot \vec{v}_1 \hat{n} \cdot \vec{S}_1 + \frac{22}{3} (\hat{n} \cdot \vec{v}_1)^2 \vec{S}_1 \cdot \vec{v}_2 \hat{n} \cdot \vec{S}_1 + \frac{20}{3} \hat{n} \cdot \vec{v}_1 \hat{n} \cdot \vec{v}_2 \vec{S}_1 \cdot \vec{v}_2 \hat{n} \cdot \vec{S}_1 + \\
& \frac{4}{3} (\hat{n} \cdot \vec{v}_2)^2 \vec{S}_1 \cdot \vec{a}_1 \hat{n} \cdot \vec{S}_1 + \frac{14}{3} \hat{n} \cdot \vec{v}_1 \hat{n} \cdot \vec{v}_2 \vec{S}_1 \cdot \vec{a}_1 \hat{n} \cdot \vec{S}_1 - \frac{10}{3} (\hat{n} \cdot \vec{v}_1)^2 \vec{S}_1 \cdot \vec{a}_2 \hat{n} \cdot \vec{S}_1 - \\
& \frac{14}{3} \hat{n} \cdot \vec{a}_2 \hat{n} \cdot \vec{v}_1 \vec{S}_1 \cdot \vec{v}_1 \hat{n} \cdot \vec{S}_1 + \frac{14}{3} \hat{n} \cdot \vec{a}_1 \hat{n} \cdot \vec{v}_2 \vec{S}_1 \cdot \vec{v}_1 \hat{n} \cdot \vec{S}_1 - \frac{7}{6} \vec{a}_1 \cdot \vec{v}_2 \vec{S}_1 \cdot \vec{v}_1 \hat{n} \cdot \vec{S}_1 + \frac{20}{3} \hat{n} \cdot \vec{a}_1 \hat{n} \cdot \vec{v}_1 \vec{S}_1 \cdot \vec{v}_2 \hat{n} \cdot \vec{S}_1 + \\
& \frac{20}{3} \hat{n} \cdot \vec{a}_1 \hat{n} \cdot \vec{v}_2 \vec{S}_1 \cdot \vec{v}_2 \hat{n} \cdot \vec{S}_1 - \frac{5}{3} \vec{a}_1 \cdot \vec{v}_2 \vec{S}_1 \cdot \vec{v}_2 \hat{n} \cdot \vec{S}_1 - \frac{5}{3} \vec{S}_1 \cdot \vec{v}_2 \vec{v}_1 \cdot \vec{a}_1 \hat{n} \cdot \vec{S}_1 + \frac{7}{6} \vec{S}_1 \cdot \vec{v}_1 \vec{v}_1 \cdot \vec{a}_2 \hat{n} \cdot \vec{S}_1 + \\
& \frac{22}{3} \hat{n} \cdot \vec{S}_1 \hat{n} \cdot \vec{v}_2 \vec{v}_1 \cdot \vec{v}_1 \hat{n} \cdot \vec{S}_1 - \frac{11}{6} \vec{S}_1 \cdot \vec{v}_2 \vec{v}_1 \cdot \vec{v}_1 \hat{n} \cdot \vec{S}_1 + \frac{5}{6} \vec{S}_1 \cdot \vec{a}_2 \vec{v}_1 \cdot \vec{v}_1 \hat{n} \cdot \vec{S}_1 + \frac{44}{3} \hat{n} \cdot \vec{S}_1 \hat{n} \cdot \vec{v}_1 \vec{v}_1 \cdot \vec{v}_2 \hat{n} \cdot \vec{S}_1 +
\end{aligned}$$

[illegible]

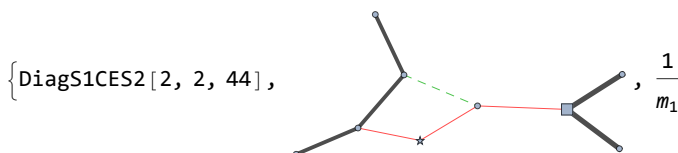

$$G^2 \left( \frac{1}{r^2} \left( \frac{8}{3} (\hat{n} \cdot \vec{v}_2)^2 \left( \hat{n} \cdot \vec{S}_1 \right)^2 - \frac{8}{3} \vec{v}_2 \cdot \vec{v}_2 \left( \hat{n} \cdot \vec{S}_1 \right)^2 - \frac{8}{3} \hat{n} \cdot \vec{a}_2 \hat{n} \cdot \vec{S}_1 \hat{n} \cdot \vec{v}_2 \hat{n} \cdot \vec{S}_1 - \frac{8}{3} \hat{n} \cdot \vec{v}_2 \vec{S}_1 \cdot \vec{v}_2 \hat{n} \cdot \vec{S}_1 + \right.$$



$$\begin{aligned}
& 18 \left( \hat{n} \cdot \vec{S}_1 \right)^2 \vec{v}_2 \cdot \vec{v}_2 \left( \hat{n} \cdot \vec{v}_2 \right)^2 + 4 \vec{S}_1 \cdot \vec{S}_1 \vec{v}_2 \cdot \vec{v}_2 \left( \hat{n} \cdot \vec{v}_2 \right)^2 + 6 \hat{n} \cdot \vec{v}_1 \left( \vec{S}_1 \cdot \vec{v}_2 \right)^2 \hat{n} \cdot \vec{v}_2 - \\
& 32 \hat{n} \cdot \vec{S}_1 \left( \hat{n} \cdot \vec{v}_1 \right)^2 \vec{S}_1 \cdot \vec{v}_2 \hat{n} \cdot \vec{v}_2 + \frac{32}{3} \hat{n} \cdot \vec{v}_1 \vec{S}_1 \cdot \vec{v}_1 \vec{S}_1 \cdot \vec{v}_2 \hat{n} \cdot \vec{v}_2 + \frac{16}{3} \hat{n} \cdot \vec{S}_1 \vec{S}_1 \cdot \vec{v}_2 \vec{v}_1 \cdot \vec{v}_1 \hat{n} \cdot \vec{v}_2 - \\
& 32 \left( \hat{n} \cdot \vec{S}_1 \right)^2 \hat{n} \cdot \vec{v}_1 \vec{v}_1 \cdot \vec{v}_2 \hat{n} \cdot \vec{v}_2 - \frac{32}{3} \hat{n} \cdot \vec{v}_1 \vec{S}_1 \cdot \vec{S}_1 \vec{v}_1 \cdot \vec{v}_2 \hat{n} \cdot \vec{v}_2 + \frac{32}{3} \hat{n} \cdot \vec{S}_1 \vec{S}_1 \cdot \vec{v}_1 \vec{v}_1 \cdot \vec{v}_2 \hat{n} \cdot \vec{v}_2 + \\
& 12 \hat{n} \cdot \vec{S}_1 \vec{S}_1 \cdot \vec{v}_2 \vec{v}_1 \cdot \vec{v}_2 \hat{n} \cdot \vec{v}_2 - 36 \left( \hat{n} \cdot \vec{S}_1 \right)^2 \hat{n} \cdot \vec{v}_1 \vec{v}_2 \cdot \vec{v}_2 \hat{n} \cdot \vec{v}_2 - 6 \hat{n} \cdot \vec{v}_1 \vec{S}_1 \cdot \vec{S}_1 \vec{v}_2 \cdot \vec{v}_2 \hat{n} \cdot \vec{v}_2 + \\
& 12 \hat{n} \cdot \vec{S}_1 \vec{S}_1 \cdot \vec{v}_1 \vec{v}_2 \cdot \vec{v}_2 \hat{n} \cdot \vec{v}_2 - 12 \hat{n} \cdot \vec{S}_1 \vec{S}_1 \cdot \vec{v}_2 \vec{v}_2 \cdot \vec{v}_2 \hat{n} \cdot \vec{v}_2 + \frac{8}{3} \left( \hat{n} \cdot \vec{v}_1 \right)^2 \left( \vec{S}_1 \cdot \vec{v}_2 \right)^2 + \\
& \frac{8}{3} \left( \hat{n} \cdot \vec{S}_1 \right)^2 \left( \vec{v}_1 \cdot \vec{v}_2 \right)^2 + \frac{4}{3} \vec{S}_1 \cdot \vec{S}_1 \left( \vec{v}_1 \cdot \vec{v}_2 \right)^2 - 2 \left( \hat{n} \cdot \vec{S}_1 \right)^2 \left( \vec{v}_2 \cdot \vec{v}_2 \right)^2 - \frac{1}{2} \vec{S}_1 \cdot \vec{S}_1 \left( \vec{v}_2 \cdot \vec{v}_2 \right)^2 - \\
& \frac{2}{3} \left( \vec{S}_1 \cdot \vec{v}_2 \right)^2 \vec{v}_1 \cdot \vec{v}_1 - \frac{3}{2} \left( \vec{S}_1 \cdot \vec{v}_2 \right)^2 \vec{v}_1 \cdot \vec{v}_2 + \frac{32}{3} \hat{n} \cdot \vec{S}_1 \hat{n} \cdot \vec{v}_1 \vec{S}_1 \cdot \vec{v}_2 \vec{v}_1 \cdot \vec{v}_2 - \frac{8}{3} \vec{S}_1 \cdot \vec{v}_1 \vec{S}_1 \cdot \vec{v}_2 \vec{v}_1 \cdot \vec{v}_2 - \\
& 32 \left( \hat{n} \cdot \vec{S}_1 \right)^2 \left( \hat{n} \cdot \vec{v}_1 \right)^2 \vec{v}_2 \cdot \vec{v}_2 - \frac{8}{3} \left( \vec{S}_1 \cdot \vec{v}_1 \right)^2 \vec{v}_2 \cdot \vec{v}_2 + \frac{3}{2} \left( \vec{S}_1 \cdot \vec{v}_2 \right)^2 \vec{v}_2 \cdot \vec{v}_2 - \frac{8}{3} \left( \hat{n} \cdot \vec{v}_1 \right)^2 \vec{S}_1 \cdot \vec{S}_1 \vec{v}_2 \cdot \vec{v}_2 + \\
& \frac{64}{3} \hat{n} \cdot \vec{S}_1 \hat{n} \cdot \vec{v}_1 \vec{S}_1 \cdot \vec{v}_1 \vec{v}_2 \cdot \vec{v}_2 + 12 \hat{n} \cdot \vec{S}_1 \hat{n} \cdot \vec{v}_1 \vec{S}_1 \cdot \vec{v}_2 \vec{v}_2 \cdot \vec{v}_2 - 3 \vec{S}_1 \cdot \vec{v}_1 \vec{S}_1 \cdot \vec{v}_2 \vec{v}_2 \cdot \vec{v}_2 + \frac{16}{3} \left( \hat{n} \cdot \vec{S}_1 \right)^2 \vec{v}_1 \cdot \vec{v}_1 \vec{v}_2 \cdot \vec{v}_2 + \\
& \frac{2}{3} \vec{S}_1 \cdot \vec{S}_1 \vec{v}_1 \cdot \vec{v}_1 \vec{v}_2 \cdot \vec{v}_2 + 6 \left( \hat{n} \cdot \vec{S}_1 \right)^2 \vec{v}_1 \cdot \vec{v}_2 \vec{v}_2 \cdot \vec{v}_2 + \frac{3}{2} \vec{S}_1 \cdot \vec{S}_1 \vec{v}_1 \cdot \vec{v}_2 \vec{v}_2 \cdot \vec{v}_2 \Big) \Big) m_{\text{ES}^2}^2 \Big\}
\end{aligned}$$

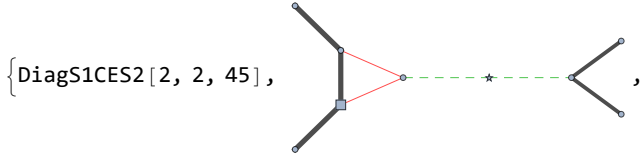

$$\begin{aligned}
& G^2 \left( \frac{1}{r} \left( -\frac{1}{6} \hat{n} \cdot \vec{a}_2 \left( \hat{n} \cdot \vec{S}_1 \right)^2 + \frac{2}{3} \vec{S}_1 \cdot \vec{a}_2 \hat{n} \cdot \vec{S}_1 - \frac{1}{6} \hat{n} \cdot \vec{S}_1 \hat{n} \cdot \vec{a}_2 \hat{n} \cdot \vec{S}_1 - \right. \right. \\
& \left. \frac{1}{6} \hat{n} \cdot \vec{a}_2 \vec{S}_1 \cdot \vec{S}_1 + \frac{1}{3} \hat{n} \cdot \vec{S}_1 \vec{S}_1 \cdot \vec{a}_2 - \frac{1}{6} \hat{n} \cdot \vec{a}_2 \vec{S}_1 \cdot \vec{S}_1 + \frac{1}{3} \hat{n} \cdot \vec{S}_1 \vec{S}_1 \cdot \vec{a}_2 \right) + \frac{1}{r^2} \\
& \left( -\frac{2}{3} \left( \hat{n} \cdot \vec{v}_2 \right)^2 \left( \hat{n} \cdot \vec{S}_1 \right)^2 + \frac{1}{6} \vec{v}_2 \cdot \vec{v}_2 \left( \hat{n} \cdot \vec{S}_1 \right)^2 + \frac{3}{2} \hat{n} \cdot \vec{a}_2 \hat{n} \cdot \vec{S}_1 \hat{n} \cdot \vec{v}_1 \hat{n} \cdot \vec{S}_1 + \frac{5}{3} \hat{n} \cdot \vec{v}_2 \vec{S}_1 \cdot \vec{v}_2 \hat{n} \cdot \vec{S}_1 - \hat{n} \cdot \vec{v}_1 \right. \\
& \left. \vec{S}_1 \cdot \vec{a}_2 \hat{n} \cdot \vec{S}_1 - \frac{1}{2} \hat{n} \cdot \vec{a}_2 \vec{S}_1 \cdot \vec{v}_1 \hat{n} \cdot \vec{S}_1 - \hat{n} \cdot \vec{S}_1 \vec{v}_1 \cdot \vec{a}_2 \hat{n} \cdot \vec{S}_1 + \frac{5}{12} \hat{n} \cdot \vec{a}_1 \hat{n} \cdot \vec{a}_2 \left( \hat{n} \cdot \vec{S}_1 \right)^2 - \frac{2}{3} \hat{n} \cdot \vec{S}_1 \hat{n} \cdot \vec{S}_1 \left( \hat{n} \cdot \vec{v}_2 \right)^2 - \right. \\
& \left. \frac{2}{3} \left( \vec{S}_1 \cdot \vec{v}_2 \right)^2 - \frac{1}{3} \left( \hat{n} \cdot \vec{v}_2 \right)^2 \vec{S}_1 \cdot \vec{S}_1 - \hat{n} \cdot \vec{S}_1 \hat{n} \cdot \vec{v}_1 \vec{S}_1 \cdot \vec{a}_2 - \frac{1}{2} \hat{n} \cdot \vec{a}_2 \hat{n} \cdot \vec{S}_1 \vec{S}_1 \cdot \vec{v}_1 + \frac{5}{6} \hat{n} \cdot \vec{S}_1 \hat{n} \cdot \vec{v}_2 \vec{S}_1 \cdot \vec{v}_2 - \right. \\
& \left. \frac{5}{12} \left( \hat{n} \cdot \vec{S}_1 \right)^2 \vec{a}_1 \cdot \vec{a}_2 + \frac{1}{2} \hat{n} \cdot \vec{a}_2 \hat{n} \cdot \vec{v}_1 \vec{S}_1 \cdot \vec{S}_1 - \frac{1}{3} \left( \hat{n} \cdot \vec{v}_2 \right)^2 \vec{S}_1 \cdot \vec{S}_1 - \frac{1}{3} \hat{n} \cdot \vec{a}_2 \hat{n} \cdot \vec{S}_1 \vec{S}_1 \cdot \vec{a}_1 - \frac{1}{3} \hat{n} \cdot \vec{a}_1 \hat{n} \cdot \vec{S}_1 \vec{S}_1 \cdot \vec{a}_2 + \right. \\
& \left. \frac{1}{2} \vec{S}_1 \cdot \vec{v}_1 \vec{S}_1 \cdot \vec{a}_2 + \frac{1}{6} \vec{S}_1 \cdot \vec{a}_1 \vec{S}_1 \cdot \vec{a}_2 + \frac{1}{12} \hat{n} \cdot \vec{a}_1 \hat{n} \cdot \vec{a}_2 \vec{S}_1 \cdot \vec{S}_1 + \frac{1}{12} \vec{a}_1 \cdot \vec{a}_2 \vec{S}_1 \cdot \vec{S}_1 + \frac{1}{2} \vec{S}_1 \cdot \vec{a}_2 \vec{S}_1 \cdot \vec{v}_1 + \right. \\
& \left. \frac{5}{6} \hat{n} \cdot \vec{S}_1 \hat{n} \cdot \vec{v}_2 \vec{S}_1 \cdot \vec{v}_2 - \frac{2}{3} \vec{S}_1 \cdot \vec{v}_2 \vec{S}_1 \cdot \vec{v}_2 + \frac{1}{6} \hat{n} \cdot \vec{S}_1 \hat{n} \cdot \vec{S}_1 \vec{v}_2 \cdot \vec{v}_2 + \frac{1}{6} \vec{S}_1 \cdot \vec{S}_1 \vec{v}_2 \cdot \vec{v}_2 + \frac{1}{6} \vec{S}_1 \cdot \vec{S}_1 \vec{v}_2 \cdot \vec{v}_2 \right) + \\
& \frac{1}{r^3} \left( -\frac{5}{2} \hat{n} \cdot \vec{a}_2 \left( \hat{n} \cdot \vec{v}_1 \right)^2 \left( \hat{n} \cdot \vec{S}_1 \right)^2 + \frac{5}{2} \hat{n} \cdot \vec{a}_1 \left( \hat{n} \cdot \vec{v}_2 \right)^2 \left( \hat{n} \cdot \vec{S}_1 \right)^2 - \frac{25}{12} \hat{n} \cdot \vec{v}_2 \vec{a}_1 \cdot \vec{v}_2 \left( \hat{n} \cdot \vec{S}_1 \right)^2 + \right. \\
& \left. \frac{25}{12} \hat{n} \cdot \vec{v}_1 \vec{v}_1 \cdot \vec{a}_2 \left( \hat{n} \cdot \vec{S}_1 \right)^2 + \frac{5}{12} \hat{n} \cdot \vec{a}_2 \vec{v}_1 \cdot \vec{v}_1 \left( \hat{n} \cdot \vec{S}_1 \right)^2 - \frac{5}{12} \hat{n} \cdot \vec{a}_1 \vec{v}_2 \cdot \vec{v}_2 \left( \hat{n} \cdot \vec{S}_1 \right)^2 + \right. \\
& \left. 9 \hat{n} \cdot \vec{S}_1 \hat{n} \cdot \vec{v}_1 \left( \hat{n} \cdot \vec{v}_2 \right)^2 \hat{n} \cdot \vec{S}_1 - 2 \left( \hat{n} \cdot \vec{v}_2 \right)^2 \vec{S}_1 \cdot \vec{v}_1 \hat{n} \cdot \vec{S}_1 - \frac{11}{2} \hat{n} \cdot \vec{v}_1 \hat{n} \cdot \vec{v}_2 \vec{S}_1 \cdot \vec{v}_2 \hat{n} \cdot \vec{S}_1 - \right. \\
& \left. \frac{4}{3} \left( \hat{n} \cdot \vec{v}_2 \right)^2 \vec{S}_1 \cdot \vec{a}_1 \hat{n} \cdot \vec{S}_1 + \frac{4}{3} \left( \hat{n} \cdot \vec{v}_1 \right)^2 \vec{S}_1 \cdot \vec{a}_2 \hat{n} \cdot \vec{S}_1 + \frac{13}{6} \hat{n} \cdot \vec{a}_2 \hat{n} \cdot \vec{v}_1 \vec{S}_1 \cdot \vec{v}_1 \hat{n} \cdot \vec{S}_1 - \frac{13}{6} \hat{n} \cdot \vec{a}_1 \hat{n} \cdot \vec{v}_2 \vec{S}_1 \cdot \vec{v}_2 \hat{n} \cdot \vec{S}_1 + \right. \\
& \left. \frac{7}{6} \vec{a}_1 \cdot \vec{v}_2 \vec{S}_1 \cdot \vec{v}_2 \hat{n} \cdot \vec{S}_1 - \frac{7}{6} \vec{S}_1 \cdot \vec{v}_1 \vec{v}_1 \cdot \vec{a}_2 \hat{n} \cdot \vec{S}_1 - \frac{1}{3} \vec{S}_1 \cdot \vec{a}_2 \vec{v}_1 \cdot \vec{v}_1 \hat{n} \cdot \vec{S}_1 - \frac{11}{2} \hat{n} \cdot \vec{S}_1 \hat{n} \cdot \vec{v}_2 \vec{v}_1 \cdot \vec{v}_2 \hat{n} \cdot \vec{S}_1 + \right. \\
& \left. 2 \vec{S}_1 \cdot \vec{v}_2 \vec{v}_1 \cdot \vec{v}_2 \hat{n} \cdot \vec{S}_1 - \frac{3}{2} \hat{n} \cdot \vec{S}_1 \hat{n} \cdot \vec{v}_1 \vec{v}_2 \cdot \vec{v}_2 \hat{n} \cdot \vec{S}_1 + \frac{1}{2} \vec{S}_1 \cdot \vec{v}_1 \vec{v}_2 \cdot \vec{v}_2 \hat{n} \cdot \vec{S}_1 + \frac{1}{3} \vec{S}_1 \cdot \vec{a}_1 \vec{v}_2 \cdot \vec{v}_2 \hat{n} \cdot \vec{S}_1 - \right.
\end{aligned}$$

$$\begin{aligned}
& \frac{1}{3} \hat{n} \cdot \vec{a}_2 \left( \vec{S}_1 \cdot \vec{v}_1 \right)^2 + \frac{1}{3} \hat{n} \cdot \vec{a}_1 \left( \vec{S}_1 \cdot \vec{v}_2 \right)^2 + 2 \hat{n} \cdot \vec{v}_1 \left( \hat{n} \cdot \vec{v}_2 \right)^2 \vec{S}_1 \cdot \vec{S}_1 - \frac{1}{3} \hat{n} \cdot \vec{a}_2 \left( \hat{n} \cdot \vec{v}_1 \right)^2 \vec{S}_1 \cdot \vec{S}_1 + \\
& \frac{1}{3} \hat{n} \cdot \vec{a}_1 \left( \hat{n} \cdot \vec{v}_2 \right)^2 \vec{S}_1 \cdot \vec{S}_1 + \frac{1}{12} \hat{n} \cdot \vec{v}_2 \vec{a}_1 \cdot \vec{v}_2 \vec{S}_1 \cdot \vec{S}_1 - 2 \hat{n} \cdot \vec{S}_1 \left( \hat{n} \cdot \vec{v}_2 \right)^2 \vec{S}_1 \cdot \vec{v}_1 + \frac{3}{2} \hat{n} \cdot \vec{v}_2 \vec{S}_1 \cdot \vec{v}_2 \vec{S}_1 \cdot \vec{v}_1 - \\
& \frac{2}{3} \hat{n} \cdot \vec{v}_1 \vec{S}_1 \cdot \vec{a}_2 \vec{S}_1 \cdot \vec{v}_1 - \frac{11}{2} \hat{n} \cdot \vec{S}_1 \hat{n} \cdot \vec{v}_1 \hat{n} \cdot \vec{v}_2 \vec{S}_1 \cdot \vec{v}_2 + \frac{3}{2} \hat{n} \cdot \vec{v}_2 \vec{S}_1 \cdot \vec{v}_1 \vec{S}_1 \cdot \vec{v}_2 + 2 \hat{n} \cdot \vec{v}_1 \vec{S}_1 \cdot \vec{v}_2 \vec{S}_1 \cdot \vec{v}_2 + \\
& \frac{2}{3} \hat{n} \cdot \vec{v}_2 \vec{S}_1 \cdot \vec{a}_1 \vec{S}_1 \cdot \vec{v}_2 - \frac{1}{12} \hat{n} \cdot \vec{v}_1 \vec{S}_1 \cdot \vec{S}_1 \vec{v}_1 \cdot \vec{a}_2 + \frac{1}{12} \hat{n} \cdot \vec{a}_2 \vec{S}_1 \cdot \vec{S}_1 \vec{v}_1 \cdot \vec{v}_1 - \frac{1}{2} \hat{n} \cdot \vec{v}_2 \vec{S}_1 \cdot \vec{S}_1 \vec{v}_1 \cdot \vec{v}_2 + \\
& 2 \hat{n} \cdot \vec{S}_1 \vec{S}_1 \cdot \vec{v}_2 \vec{v}_1 \cdot \vec{v}_2 - \frac{1}{2} \hat{n} \cdot \vec{v}_1 \vec{S}_1 \cdot \vec{S}_1 \vec{v}_2 \cdot \vec{v}_2 - \frac{1}{12} \hat{n} \cdot \vec{a}_1 \vec{S}_1 \cdot \vec{S}_1 \vec{v}_2 \cdot \vec{v}_2 + \frac{1}{2} \hat{n} \cdot \vec{S}_1 \vec{S}_1 \cdot \vec{v}_1 \vec{v}_2 \cdot \vec{v}_2 \Big) + \\
& \frac{1}{r^4} \left( -20 \left( \hat{n} \cdot \vec{v}_1 \right)^2 \left( \hat{n} \cdot \vec{v}_2 \right)^2 \left( \hat{n} \cdot \vec{S}_1 \right)^2 - \frac{25}{12} \left( \vec{v}_1 \cdot \vec{v}_2 \right)^2 \left( \hat{n} \cdot \vec{S}_1 \right)^2 + \frac{5}{2} \left( \hat{n} \cdot \vec{v}_2 \right)^2 \vec{v}_1 \cdot \vec{v}_1 \left( \hat{n} \cdot \vec{S}_1 \right)^2 + \right. \\
& \frac{35}{2} \hat{n} \cdot \vec{v}_1 \hat{n} \cdot \vec{v}_2 \vec{v}_1 \cdot \vec{v}_2 \left( \hat{n} \cdot \vec{S}_1 \right)^2 + \frac{5}{2} \left( \hat{n} \cdot \vec{v}_1 \right)^2 \vec{v}_2 \cdot \vec{v}_2 \left( \hat{n} \cdot \vec{S}_1 \right)^2 - \frac{5}{12} \vec{v}_1 \cdot \vec{v}_1 \vec{v}_2 \cdot \vec{v}_2 \left( \hat{n} \cdot \vec{S}_1 \right)^2 + \\
& 13 \hat{n} \cdot \vec{v}_1 \left( \hat{n} \cdot \vec{v}_2 \right)^2 \vec{S}_1 \cdot \vec{v}_1 \hat{n} \cdot \vec{S}_1 + 13 \left( \hat{n} \cdot \vec{v}_1 \right)^2 \hat{n} \cdot \vec{v}_2 \vec{S}_1 \cdot \vec{v}_2 \hat{n} \cdot \vec{S}_1 - \frac{13}{6} \hat{n} \cdot \vec{v}_2 \vec{S}_1 \cdot \vec{v}_2 \vec{v}_1 \cdot \vec{v}_1 \hat{n} \cdot \vec{S}_1 - \\
& \frac{41}{6} \hat{n} \cdot \vec{v}_2 \vec{S}_1 \cdot \vec{v}_1 \vec{v}_1 \cdot \vec{v}_2 \hat{n} \cdot \vec{S}_1 - \frac{41}{6} \hat{n} \cdot \vec{v}_1 \vec{S}_1 \cdot \vec{v}_2 \vec{v}_1 \cdot \vec{v}_2 \hat{n} \cdot \vec{S}_1 - \frac{13}{6} \hat{n} \cdot \vec{v}_1 \vec{S}_1 \cdot \vec{v}_1 \vec{v}_2 \cdot \vec{v}_2 \hat{n} \cdot \vec{S}_1 - \\
& \frac{4}{3} \left( \hat{n} \cdot \vec{v}_2 \right)^2 \left( \vec{S}_1 \cdot \vec{v}_1 \right)^2 - \frac{4}{3} \left( \hat{n} \cdot \vec{v}_1 \right)^2 \left( \vec{S}_1 \cdot \vec{v}_2 \right)^2 + \frac{1}{12} \vec{S}_1 \cdot \vec{S}_1 \left( \vec{v}_1 \cdot \vec{v}_2 \right)^2 - 2 \left( \hat{n} \cdot \vec{v}_1 \right)^2 \left( \hat{n} \cdot \vec{v}_2 \right)^2 \vec{S}_1 \cdot \vec{S}_1 - \\
& \frac{29}{6} \hat{n} \cdot \vec{v}_1 \hat{n} \cdot \vec{v}_2 \vec{S}_1 \cdot \vec{v}_1 \vec{S}_1 \cdot \vec{v}_2 + \frac{1}{3} \left( \vec{S}_1 \cdot \vec{v}_2 \right)^2 \vec{v}_1 \cdot \vec{v}_1 + \frac{1}{3} \left( \hat{n} \cdot \vec{v}_2 \right)^2 \vec{S}_1 \cdot \vec{S}_1 \vec{v}_1 \cdot \vec{v}_1 + \frac{1}{3} \hat{n} \cdot \vec{v}_1 \hat{n} \cdot \vec{v}_2 \vec{S}_1 \cdot \vec{S}_1 \vec{v}_1 \cdot \vec{v}_2 + \\
& \left. \frac{11}{6} \vec{S}_1 \cdot \vec{v}_1 \vec{S}_1 \cdot \vec{v}_2 \vec{v}_1 \cdot \vec{v}_2 + \frac{1}{3} \left( \vec{S}_1 \cdot \vec{v}_1 \right)^2 \vec{v}_2 \cdot \vec{v}_2 + \frac{1}{3} \left( \hat{n} \cdot \vec{v}_1 \right)^2 \vec{S}_1 \cdot \vec{S}_1 \vec{v}_2 \cdot \vec{v}_2 - \frac{1}{12} \vec{S}_1 \cdot \vec{S}_1 \vec{v}_1 \cdot \vec{v}_1 \vec{v}_2 \cdot \vec{v}_2 \right) \Big) m_2 C_{ES^2 1} \}
\end{aligned}$$

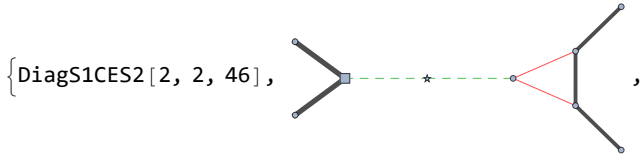

$$\begin{aligned}
& \frac{1}{m_1} G^2 \left( \frac{1}{r} \left( -\frac{1}{3} \hat{n} \cdot \vec{a}_2 \left( \hat{n} \cdot \vec{S}_1 \right)^2 + \frac{5}{6} \vec{S}_1 \cdot \vec{a}_2 \hat{n} \cdot \vec{S}_1 - \frac{1}{3} \hat{n} \cdot \vec{S}_1 \hat{n} \cdot \vec{a}_2 \hat{n} \cdot \vec{S}_1 - \right. \right. \\
& \left. \frac{5}{6} \hat{n} \cdot \vec{a}_2 \vec{S}_1 \cdot \vec{S}_1 + \frac{5}{12} \hat{n} \cdot \vec{S}_1 \vec{S}_1 \cdot \vec{a}_2 - \frac{5}{6} \hat{n} \cdot \vec{a}_2 \vec{S}_1 \cdot \vec{S}_1 + \frac{5}{12} \hat{n} \cdot \vec{S}_1 \vec{S}_1 \cdot \vec{a}_2 \right) + \frac{1}{r^2} \\
& \left( -\frac{4}{3} \left( \hat{n} \cdot \vec{v}_2 \right)^2 \left( \hat{n} \cdot \vec{S}_1 \right)^2 + \frac{1}{3} \vec{v}_2 \cdot \vec{v}_2 \left( \hat{n} \cdot \vec{S}_1 \right)^2 + \frac{8}{3} \hat{n} \cdot \vec{a}_2 \hat{n} \cdot \vec{S}_1 \hat{n} \cdot \vec{v}_1 \hat{n} \cdot \vec{S}_1 + \frac{7}{3} \hat{n} \cdot \vec{v}_2 \vec{S}_1 \cdot \vec{v}_2 \hat{n} \cdot \vec{S}_1 - \right. \\
& \frac{7}{6} \hat{n} \cdot \vec{v}_1 \vec{S}_1 \cdot \vec{a}_2 \hat{n} \cdot \vec{S}_1 - \frac{2}{3} \hat{n} \cdot \vec{a}_2 \vec{S}_1 \cdot \vec{v}_1 \hat{n} \cdot \vec{S}_1 - \frac{5}{3} \hat{n} \cdot \vec{S}_1 \vec{v}_1 \cdot \vec{a}_2 \hat{n} \cdot \vec{S}_1 + \frac{2}{3} \hat{n} \cdot \vec{a}_1 \hat{n} \cdot \vec{a}_2 \left( \hat{n} \cdot \vec{S}_1 \right)^2 - \\
& \frac{4}{3} \hat{n} \cdot \vec{S}_1 \hat{n} \cdot \vec{S}_1 \left( \hat{n} \cdot \vec{v}_2 \right)^2 - \frac{5}{6} \left( \vec{S}_1 \cdot \vec{v}_2 \right)^2 - \frac{5}{3} \left( \hat{n} \cdot \vec{v}_2 \right)^2 \vec{S}_1 \cdot \vec{S}_1 - \frac{7}{6} \hat{n} \cdot \vec{S}_1 \hat{n} \cdot \vec{v}_1 \vec{S}_1 \cdot \vec{a}_2 - \frac{2}{3} \hat{n} \cdot \vec{a}_2 \hat{n} \cdot \vec{S}_1 \vec{S}_1 \cdot \vec{v}_1 + \\
& \frac{7}{6} \hat{n} \cdot \vec{S}_1 \hat{n} \cdot \vec{v}_2 \vec{S}_1 \cdot \vec{v}_2 - \frac{2}{3} \left( \hat{n} \cdot \vec{S}_1 \right)^2 \vec{a}_1 \cdot \vec{a}_2 + \frac{7}{3} \hat{n} \cdot \vec{a}_2 \hat{n} \cdot \vec{v}_1 \vec{S}_1 \cdot \vec{S}_1 - \frac{5}{3} \left( \hat{n} \cdot \vec{v}_2 \right)^2 \vec{S}_1 \cdot \vec{S}_1 - \\
& \frac{1}{3} \hat{n} \cdot \vec{a}_2 \hat{n} \cdot \vec{S}_1 \vec{S}_1 \cdot \vec{a}_1 - \frac{1}{3} \hat{n} \cdot \vec{a}_1 \hat{n} \cdot \vec{S}_1 \vec{S}_1 \cdot \vec{a}_2 + \frac{7}{12} \vec{S}_1 \cdot \vec{v}_1 \vec{S}_1 \cdot \vec{a}_2 + \frac{1}{6} \vec{S}_1 \cdot \vec{a}_1 \vec{S}_1 \cdot \vec{a}_2 + \\
& \frac{1}{3} \hat{n} \cdot \vec{a}_1 \hat{n} \cdot \vec{a}_2 \vec{S}_1 \cdot \vec{S}_1 - \frac{1}{6} \vec{a}_1 \cdot \vec{a}_2 \vec{S}_1 \cdot \vec{S}_1 + \frac{7}{12} \vec{S}_1 \cdot \vec{a}_2 \vec{S}_1 \cdot \vec{v}_1 + \frac{7}{6} \hat{n} \cdot \vec{S}_1 \hat{n} \cdot \vec{v}_2 \vec{S}_1 \cdot \vec{v}_2 - \\
& \left. \frac{5}{6} \vec{S}_1 \cdot \vec{v}_2 \vec{S}_1 \cdot \vec{v}_2 - \frac{7}{6} \vec{S}_1 \cdot \vec{S}_1 \vec{v}_1 \cdot \vec{a}_2 + \frac{1}{3} \hat{n} \cdot \vec{S}_1 \hat{n} \cdot \vec{S}_1 \vec{v}_2 \cdot \vec{v}_2 + \frac{5}{6} \vec{S}_1 \cdot \vec{S}_1 \vec{v}_2 \cdot \vec{v}_2 + \frac{5}{6} \vec{S}_1 \cdot \vec{S}_1 \vec{v}_2 \cdot \vec{v}_2 \right) + \\
& \frac{1}{r^3} \left( -4 \hat{n} \cdot \vec{a}_2 \left( \hat{n} \cdot \vec{v}_1 \right)^2 \left( \hat{n} \cdot \vec{S}_1 \right)^2 + 4 \hat{n} \cdot \vec{a}_1 \left( \hat{n} \cdot \vec{v}_2 \right)^2 \left( \hat{n} \cdot \vec{S}_1 \right)^2 - \frac{10}{3} \hat{n} \cdot \vec{v}_2 \vec{a}_1 \cdot \vec{v}_2 \left( \hat{n} \cdot \vec{S}_1 \right)^2 + \right. \\
& \left. \frac{10}{3} \hat{n} \cdot \vec{v}_1 \vec{v}_1 \cdot \vec{a}_2 \left( \hat{n} \cdot \vec{S}_1 \right)^2 + \frac{2}{3} \hat{n} \cdot \vec{a}_2 \vec{v}_1 \cdot \vec{v}_1 \left( \hat{n} \cdot \vec{S}_1 \right)^2 - \frac{2}{3} \hat{n} \cdot \vec{a}_1 \vec{v}_2 \cdot \vec{v}_2 \left( \hat{n} \cdot \vec{S}_1 \right)^2 + \right.
\end{aligned}$$

$$\begin{aligned}
& 16 \hat{n} \cdot \vec{S}_1 \hat{n} \cdot \vec{v}_1 (\hat{n} \cdot \vec{v}_2)^2 \hat{n} \cdot \vec{S}_1 - \frac{8}{3} (\hat{n} \cdot \vec{v}_2)^2 \vec{S}_1 \cdot \vec{v}_1 \hat{n} \cdot \vec{S}_1 - \frac{22}{3} \hat{n} \cdot \vec{v}_1 \hat{n} \cdot \vec{v}_2 \vec{S}_1 \cdot \vec{v}_2 \hat{n} \cdot \vec{S}_1 - \\
& \frac{4}{3} (\hat{n} \cdot \vec{v}_2)^2 \vec{S}_1 \cdot \vec{a}_1 \hat{n} \cdot \vec{S}_1 + \frac{4}{3} (\hat{n} \cdot \vec{v}_1)^2 \vec{S}_1 \cdot \vec{a}_2 \hat{n} \cdot \vec{S}_1 + \frac{8}{3} \hat{n} \cdot \vec{a}_2 \hat{n} \cdot \vec{v}_1 \vec{S}_1 \cdot \vec{v}_1 \hat{n} \cdot \vec{S}_1 - \frac{8}{3} \hat{n} \cdot \vec{a}_1 \hat{n} \cdot \vec{v}_2 \vec{S}_1 \cdot \vec{v}_2 \hat{n} \cdot \vec{S}_1 + \\
& \frac{5}{3} \vec{a}_1 \cdot \vec{v}_2 \vec{S}_1 \cdot \vec{v}_2 \hat{n} \cdot \vec{S}_1 - \frac{5}{3} \vec{S}_1 \cdot \vec{v}_1 \vec{v}_1 \cdot \vec{a}_2 \hat{n} \cdot \vec{S}_1 - \frac{1}{3} \vec{S}_1 \cdot \vec{a}_2 \vec{v}_1 \cdot \vec{v}_1 \hat{n} \cdot \vec{S}_1 - \frac{28}{3} \hat{n} \cdot \vec{S}_1 \hat{n} \cdot \vec{v}_2 \vec{v}_1 \cdot \vec{v}_2 \hat{n} \cdot \vec{S}_1 + \\
& \frac{17}{6} \vec{S}_1 \cdot \vec{v}_2 \vec{v}_1 \cdot \vec{v}_2 \hat{n} \cdot \vec{S}_1 - \frac{8}{3} \hat{n} \cdot \vec{S}_1 \hat{n} \cdot \vec{v}_1 \vec{v}_2 \cdot \vec{v}_2 \hat{n} \cdot \vec{S}_1 + \frac{2}{3} \vec{S}_1 \cdot \vec{v}_1 \vec{v}_2 \cdot \vec{v}_2 \hat{n} \cdot \vec{S}_1 + \frac{1}{3} \vec{S}_1 \cdot \vec{a}_1 \vec{v}_2 \cdot \vec{v}_2 \hat{n} \cdot \vec{S}_1 - \\
& \frac{1}{3} \hat{n} \cdot \vec{a}_2 (\vec{S}_1 \cdot \vec{v}_1)^2 + \frac{1}{3} \hat{n} \cdot \vec{a}_1 (\vec{S}_1 \cdot \vec{v}_2)^2 + \frac{28}{3} \hat{n} \cdot \vec{v}_1 (\hat{n} \cdot \vec{v}_2)^2 \vec{S}_1 \cdot \vec{S}_1 - \frac{4}{3} \hat{n} \cdot \vec{a}_2 (\hat{n} \cdot \vec{v}_1)^2 \vec{S}_1 \cdot \vec{S}_1 + \\
& \frac{4}{3} \hat{n} \cdot \vec{a}_1 (\hat{n} \cdot \vec{v}_2)^2 \vec{S}_1 \cdot \vec{S}_1 - \frac{2}{3} \hat{n} \cdot \vec{v}_2 \vec{a}_1 \cdot \vec{v}_2 \vec{S}_1 \cdot \vec{S}_1 - \frac{8}{3} \hat{n} \cdot \vec{S}_1 (\hat{n} \cdot \vec{v}_2)^2 \vec{S}_1 \cdot \vec{v}_1 + \frac{11}{6} \hat{n} \cdot \vec{v}_2 \vec{S}_1 \cdot \vec{v}_2 \vec{S}_1 \cdot \vec{v}_1 - \\
& \frac{2}{3} \hat{n} \cdot \vec{v}_1 \vec{S}_1 \cdot \vec{a}_2 \vec{S}_1 \cdot \vec{v}_1 - \frac{22}{3} \hat{n} \cdot \vec{S}_1 \hat{n} \cdot \vec{v}_1 \hat{n} \cdot \vec{v}_2 \vec{S}_1 \cdot \vec{v}_2 + \frac{11}{6} \hat{n} \cdot \vec{v}_2 \vec{S}_1 \cdot \vec{v}_1 \vec{S}_1 \cdot \vec{v}_2 + \frac{7}{3} \hat{n} \cdot \vec{v}_1 \vec{S}_1 \cdot \vec{v}_2 \vec{S}_1 \cdot \vec{v}_2 + \\
& \frac{2}{3} \hat{n} \cdot \vec{v}_2 \vec{S}_1 \cdot \vec{a}_1 \vec{S}_1 \cdot \vec{v}_2 + \frac{2}{3} \hat{n} \cdot \vec{v}_1 \vec{S}_1 \cdot \vec{S}_1 \vec{v}_1 \cdot \vec{a}_2 + \frac{1}{3} \hat{n} \cdot \vec{a}_2 \vec{S}_1 \cdot \vec{S}_1 \vec{v}_1 \cdot \vec{v}_1 - \frac{14}{3} \hat{n} \cdot \vec{v}_2 \vec{S}_1 \cdot \vec{S}_1 \vec{v}_1 \cdot \vec{v}_2 + \\
& \frac{17}{6} \hat{n} \cdot \vec{S}_1 \vec{S}_1 \cdot \vec{v}_2 \vec{v}_1 \cdot \vec{v}_2 - \frac{7}{3} \hat{n} \cdot \vec{v}_1 \vec{S}_1 \cdot \vec{S}_1 \vec{v}_2 \cdot \vec{v}_2 - \frac{1}{3} \hat{n} \cdot \vec{a}_1 \vec{S}_1 \cdot \vec{S}_1 \vec{v}_2 \cdot \vec{v}_2 + \frac{2}{3} \hat{n} \cdot \vec{S}_1 \vec{S}_1 \cdot \vec{v}_1 \vec{v}_2 \cdot \vec{v}_2 \Big) + \\
& \frac{1}{r^4} \left( -32 (\hat{n} \cdot \vec{v}_1)^2 (\hat{n} \cdot \vec{v}_2)^2 (\hat{n} \cdot \vec{S}_1)^2 - \frac{10}{3} (\vec{v}_1 \cdot \vec{v}_2)^2 (\hat{n} \cdot \vec{S}_1)^2 + 4 (\hat{n} \cdot \vec{v}_2)^2 \vec{v}_1 \cdot \vec{v}_1 (\hat{n} \cdot \vec{S}_1)^2 + \right. \\
& 28 \hat{n} \cdot \vec{v}_1 \hat{n} \cdot \vec{v}_2 \vec{v}_1 \cdot \vec{v}_2 (\hat{n} \cdot \vec{S}_1)^2 + 4 (\hat{n} \cdot \vec{v}_1)^2 \vec{v}_2 \cdot \vec{v}_2 (\hat{n} \cdot \vec{S}_1)^2 - \frac{2}{3} \vec{v}_1 \cdot \vec{v}_1 \vec{v}_2 \cdot \vec{v}_2 (\hat{n} \cdot \vec{S}_1)^2 + \\
& 16 \hat{n} \cdot \vec{v}_1 (\hat{n} \cdot \vec{v}_2)^2 \vec{S}_1 \cdot \vec{v}_1 \hat{n} \cdot \vec{S}_1 + 16 (\hat{n} \cdot \vec{v}_1)^2 \hat{n} \cdot \vec{v}_2 \vec{S}_1 \cdot \vec{v}_2 \hat{n} \cdot \vec{S}_1 - \frac{8}{3} \hat{n} \cdot \vec{v}_2 \vec{S}_1 \cdot \vec{v}_2 \vec{v}_1 \cdot \vec{v}_1 \hat{n} \cdot \vec{S}_1 - \\
& \frac{28}{3} \hat{n} \cdot \vec{v}_2 \vec{S}_1 \cdot \vec{v}_1 \vec{v}_1 \cdot \vec{v}_2 \hat{n} \cdot \vec{S}_1 - \frac{28}{3} \hat{n} \cdot \vec{v}_1 \vec{S}_1 \cdot \vec{v}_2 \vec{v}_1 \cdot \vec{v}_2 \hat{n} \cdot \vec{S}_1 - \frac{8}{3} \hat{n} \cdot \vec{v}_1 \vec{S}_1 \cdot \vec{v}_1 \vec{v}_2 \cdot \vec{v}_2 \hat{n} \cdot \vec{S}_1 - \\
& \frac{4}{3} (\hat{n} \cdot \vec{v}_2)^2 (\vec{S}_1 \cdot \vec{v}_1)^2 - \frac{4}{3} (\hat{n} \cdot \vec{v}_1)^2 (\vec{S}_1 \cdot \vec{v}_2)^2 - \frac{2}{3} \vec{S}_1 \cdot \vec{S}_1 (\vec{v}_1 \cdot \vec{v}_2)^2 - 8 (\hat{n} \cdot \vec{v}_1)^2 (\hat{n} \cdot \vec{v}_2)^2 \vec{S}_1 \cdot \vec{S}_1 - \\
& \frac{16}{3} \hat{n} \cdot \vec{v}_1 \hat{n} \cdot \vec{v}_2 \vec{S}_1 \cdot \vec{v}_1 \vec{S}_1 \cdot \vec{v}_2 + \frac{1}{3} (\vec{S}_1 \cdot \vec{v}_2)^2 \vec{v}_1 \cdot \vec{v}_1 + \frac{4}{3} (\hat{n} \cdot \vec{v}_2)^2 \vec{S}_1 \cdot \vec{S}_1 \vec{v}_1 \cdot \vec{v}_1 + \frac{16}{3} \hat{n} \cdot \vec{v}_1 \hat{n} \cdot \vec{v}_2 \vec{S}_1 \cdot \vec{S}_1 \vec{v}_1 \cdot \vec{v}_2 + \\
& \left. \frac{7}{3} \vec{S}_1 \cdot \vec{v}_1 \vec{S}_1 \cdot \vec{v}_2 \vec{v}_1 \cdot \vec{v}_2 + \frac{1}{3} (\vec{S}_1 \cdot \vec{v}_1)^2 \vec{v}_2 \cdot \vec{v}_2 + \frac{4}{3} (\hat{n} \cdot \vec{v}_1)^2 \vec{S}_1 \cdot \vec{S}_1 \vec{v}_2 \cdot \vec{v}_2 - \frac{1}{3} \vec{S}_1 \cdot \vec{S}_1 \vec{v}_1 \cdot \vec{v}_1 \vec{v}_2 \cdot \vec{v}_2 \right) \Big) m_{\text{ES}^2}^2 \}
\end{aligned}$$

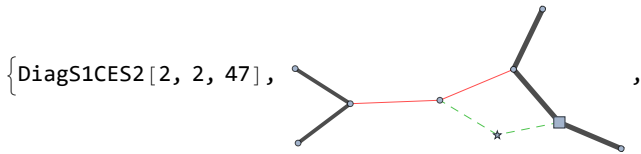

$$\begin{aligned}
& G^2 \left( \frac{1}{r} \left( \frac{2}{3} \hat{n} \cdot \vec{a}_1 (\hat{n} \cdot \vec{S}_1)^2 + \frac{2}{3} \hat{n} \cdot \vec{a}_2 (\hat{n} \cdot \vec{S}_1)^2 + \frac{1}{3} \vec{S}_1 \cdot \vec{a}_1 \hat{n} \cdot \vec{S}_1 - \frac{2}{3} \vec{S}_1 \cdot \vec{a}_2 \hat{n} \cdot \vec{S}_1 + \right. \right. \\
& \frac{2}{3} \hat{n} \cdot \vec{S}_1 \hat{n} \cdot \vec{a}_1 \hat{n} \cdot \vec{S}_1 + \frac{2}{3} \hat{n} \cdot \vec{S}_1 \hat{n} \cdot \vec{a}_2 \hat{n} \cdot \vec{S}_1 - \frac{1}{3} \hat{n} \cdot \vec{a}_1 \vec{S}_1 \cdot \vec{S}_1 - \frac{4}{3} \hat{n} \cdot \vec{a}_2 \vec{S}_1 \cdot \vec{S}_1 + \frac{1}{6} \hat{n} \cdot \vec{S}_1 \vec{S}_1 \cdot \vec{a}_1 - \\
& \left. \frac{1}{3} \hat{n} \cdot \vec{S}_1 \vec{S}_1 \cdot \vec{a}_2 - \frac{1}{3} \hat{n} \cdot \vec{a}_1 \vec{S}_1 \cdot \vec{S}_1 - \frac{4}{3} \hat{n} \cdot \vec{a}_2 \vec{S}_1 \cdot \vec{S}_1 + \frac{1}{6} \hat{n} \cdot \vec{S}_1 \vec{S}_1 \cdot \vec{a}_1 - \frac{1}{3} \hat{n} \cdot \vec{S}_1 \vec{S}_1 \cdot \vec{a}_2 \right) + \\
& \frac{1}{r^2} \left( -2 (\hat{n} \cdot \vec{v}_1)^2 (\hat{n} \cdot \vec{S}_1)^2 + \frac{8}{3} (\hat{n} \cdot \vec{v}_2)^2 (\hat{n} \cdot \vec{S}_1)^2 + \frac{2}{3} \hat{n} \cdot \vec{v}_1 \hat{n} \cdot \vec{v}_2 (\hat{n} \cdot \vec{S}_1)^2 + \vec{v}_1 \cdot \vec{v}_1 (\hat{n} \cdot \vec{S}_1)^2 - \right. \\
& \frac{1}{6} \vec{v}_1 \cdot \vec{v}_2 (\hat{n} \cdot \vec{S}_1)^2 - \frac{2}{3} \vec{v}_2 \cdot \vec{v}_2 (\hat{n} \cdot \vec{S}_1)^2 - \frac{4}{3} \hat{n} \cdot \vec{a}_1 \hat{n} \cdot \vec{S}_1 \hat{n} \cdot \vec{v}_1 \hat{n} \cdot \vec{S}_1 - \frac{4}{3} \hat{n} \cdot \vec{a}_2 \hat{n} \cdot \vec{S}_1 \hat{n} \cdot \vec{v}_1 \hat{n} \cdot \vec{S}_1 - \\
& \hat{n} \cdot \vec{v}_1 \vec{S}_1 \cdot \vec{v}_1 \hat{n} \cdot \vec{S}_1 + \frac{2}{3} \hat{n} \cdot \vec{v}_2 \vec{S}_1 \cdot \vec{v}_1 \hat{n} \cdot \vec{S}_1 - \frac{1}{3} \hat{n} \cdot \vec{v}_1 \vec{S}_1 \cdot \vec{v}_2 \hat{n} \cdot \vec{S}_1 - \frac{8}{3} \hat{n} \cdot \vec{v}_2 \vec{S}_1 \cdot \vec{v}_2 \hat{n} \cdot \vec{S}_1 - \frac{5}{12} \hat{n} \cdot \vec{v}_1 \vec{S}_1 \cdot \vec{a}_1 \hat{n} \cdot \vec{S}_1 + \\
& \left. \frac{1}{3} \hat{n} \cdot \vec{v}_1 \vec{S}_1 \cdot \vec{a}_2 \hat{n} \cdot \vec{S}_1 + \frac{13}{12} \hat{n} \cdot \vec{a}_1 \vec{S}_1 \cdot \vec{v}_1 \hat{n} \cdot \vec{S}_1 + \frac{1}{3} \hat{n} \cdot \vec{a}_2 \vec{S}_1 \cdot \vec{v}_1 \hat{n} \cdot \vec{S}_1 - \frac{1}{6} \hat{n} \cdot \vec{S}_1 \vec{v}_1 \cdot \vec{a}_1 \hat{n} \cdot \vec{S}_1 + \right.
\end{aligned}$$





[illegible]

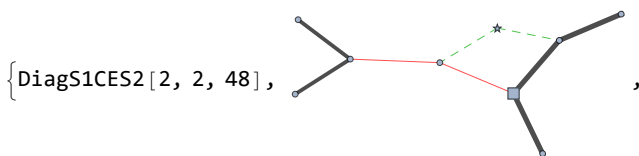

$$G^2 \left[ \frac{-2\hat{n} \cdot \vec{a}_1 \left( \hat{n} \cdot \vec{S}_1 \right)^2 + 2\vec{S}_1 \cdot \vec{a}_1 \hat{n} \cdot \vec{S}_1 - 2\hat{n} \cdot \vec{S}_1 \hat{n} \cdot \vec{a}_1 \hat{n} \cdot \vec{S}_1 + \hat{n} \cdot \vec{S}_1 \vec{S}_1 \cdot \vec{a}_1 + \hat{n} \cdot \vec{S}_1 \vec{S}_1 \cdot \vec{a}_1}{r} + \frac{1}{r^2} \right.$$
$$\begin{aligned} & \left( -2(\hat{n} \cdot \vec{v}_1)^2 \left( \hat{n} \cdot \vec{S}_1 \right)^2 + \frac{1}{2} \vec{v}_1 \cdot \vec{v}_1 \left( \hat{n} \cdot \vec{S}_1 \right)^2 + 20\hat{n} \cdot \vec{a}_1 \hat{n} \cdot \vec{S}_1 \hat{n} \cdot \vec{v}_1 \hat{n} \cdot \vec{S}_1 + 2\hat{n} \cdot \vec{a}_1 \hat{n} \cdot \vec{S}_1 \hat{n} \cdot \vec{v}_2 \hat{n} \cdot \vec{S}_1 - \right. \\ & \hat{n} \cdot \vec{v}_1 \vec{S}_1 \cdot \vec{v}_1 \hat{n} \cdot \vec{S}_1 - \frac{1}{2} \hat{n} \cdot \vec{S}_1 \vec{a}_1 \cdot \vec{v}_2 \hat{n} \cdot \vec{S}_1 - 5\hat{n} \cdot \vec{v}_1 \vec{S}_1 \cdot \vec{a}_1 \hat{n} \cdot \vec{S}_1 + \hat{n} \cdot \vec{v}_2 \vec{S}_1 \cdot \vec{a}_1 \hat{n} \cdot \vec{S}_1 - 2\hat{n} \cdot \vec{a}_1 \vec{S}_1 \cdot \vec{v}_1 \hat{n} \cdot \vec{S}_1 - \\ & \frac{1}{2} \hat{n} \cdot \vec{a}_1 \vec{S}_1 \cdot \vec{v}_2 \hat{n} \cdot \vec{S}_1 - 5\hat{n} \cdot \vec{S}_1 \vec{v}_1 \cdot \vec{a}_1 \hat{n} \cdot \vec{S}_1 + 5(\hat{n} \cdot \vec{a}_1)^2 (\hat{n} \cdot \vec{S}_1)^2 + 5\hat{n} \cdot \vec{a}_1 \hat{n} \cdot \vec{a}_2 (\hat{n} \cdot \vec{S}_1)^2 - \\ & 2\hat{n} \cdot \vec{S}_1 \hat{n} \cdot \vec{S}_1 (\hat{n} \cdot \vec{v}_1)^2 + \left( \frac{1}{\vec{S}_1 \cdot \vec{v}_1} \right)^2 + \frac{1}{2} (\vec{S}_1 \cdot \vec{a}_1)^2 + (\hat{n} \cdot \vec{v}_1)^2 \vec{S}_1 \cdot \vec{S}_1 - 5\hat{n} \cdot \vec{S}_1 \hat{n} \cdot \vec{v}_1 \vec{S}_1 \cdot \vec{a}_1 + \hat{n} \cdot \vec{S}_1 \hat{n} \cdot \vec{v}_2 \vec{S}_1 \cdot \vec{a}_1 - \\ & 2\hat{n} \cdot \vec{a}_1 \hat{n} \cdot \vec{S}_1 \vec{S}_1 \cdot \vec{v}_1 - \frac{1}{2} \hat{n} \cdot \vec{a}_1 \hat{n} \cdot \vec{S}_1 \vec{S}_1 \cdot \vec{v}_2 - \frac{1}{2} \hat{n} \cdot \vec{S}_1 \hat{n} \cdot \vec{v}_1 \vec{S}_1^2 \cdot \vec{v}_1 - \frac{5}{4} (\hat{n} \cdot \vec{S}_1)^2 \vec{a}_1 \cdot \vec{a}_1 - \frac{5}{4} (\hat{n} \cdot \vec{S}_1)^2 \vec{a}_1 \cdot \vec{a}_2 - \\ & 2\hat{n} \cdot \vec{a}_1 \hat{n} \cdot \vec{v}_1 \vec{S}_1 \cdot \vec{S}_1 - \hat{n} \cdot \vec{a}_1 \hat{n} \cdot \vec{v}_2 \vec{S}_1 \cdot \vec{S}_1 + \frac{1}{2} \vec{a}_1 \cdot \vec{v}_2 \vec{S}_1 \cdot \vec{S}_1 + (\hat{n} \cdot \vec{v}_1)^2 \vec{S}_1 \cdot \vec{S}_1 - \frac{7}{2} \hat{n} \cdot \vec{a}_1 \hat{n} \cdot \vec{S}_1 \vec{S}_1 \cdot \vec{a}_1 - \\ & \hat{n} \cdot \vec{a}_2 \hat{n} \cdot \vec{S}_1 \vec{S}_1 \cdot \vec{a}_1 + \vec{S}_1 \cdot \vec{v}_1 \vec{S}_1 \cdot \vec{a}_1 - \frac{1}{2} \vec{S}_1 \cdot \vec{v}_2 \vec{S}_1 \cdot \vec{a}_1 - \frac{5}{2} \hat{n} \cdot \vec{a}_1 \hat{n} \cdot \vec{S}_1 \vec{S}_1 \cdot \vec{a}_2 + \frac{1}{2} \vec{S}_1 \cdot \vec{a}_1 \vec{S}_1 \cdot \vec{a}_2 - \frac{1}{2} (\hat{n} \cdot \vec{a}_1)^2 \vec{S}_1 \cdot \vec{S}_1 - \\ & \frac{1}{2} \hat{n} \cdot \vec{a}_1 \hat{n} \cdot \vec{a}_2 \vec{S}_1 \cdot \vec{S}_1 + \frac{1}{4} \vec{a}_1 \cdot \vec{a}_1 \vec{S}_1 \cdot \vec{S}_1 + \frac{1}{4} \vec{a}_1 \cdot \vec{a}_2 \vec{S}_1 \cdot \vec{S}_1 - \frac{1}{2} \hat{n} \cdot \vec{S}_1 \hat{n} \cdot \vec{v}_1 \vec{S}_1 \cdot \vec{v}_1 + \vec{S}_1 \cdot \vec{a}_1 \vec{S}_1 \cdot \vec{v}_1 + \\ & \left. \vec{S}_1 \cdot \vec{v}_1 \vec{S}_1 \cdot \vec{v}_1 - \frac{1}{2} \vec{S}_1 \cdot \vec{a}_1 \vec{S}_1 \cdot \vec{v}_2 + \vec{S}_1 \cdot \vec{S}_1 \vec{v}_1 \cdot \vec{a}_1 + \frac{1}{2} \hat{n} \cdot \vec{S}_1 \hat{n} \cdot \vec{S}_1 \vec{v}_1 \cdot \vec{v}_1 - \frac{1}{2} \vec{S}_1 \cdot \vec{S}_1 \vec{v}_1 \cdot \vec{v}_1 - \frac{1}{2} \vec{S}_1 \cdot \vec{S}_1 \vec{v}_1 \cdot \vec{v}_1 \right) + \frac{1}{r^3} \end{aligned}$$
$$\begin{aligned} & \left( 20\hat{n} \cdot \vec{S}_1 \hat{n} \cdot \vec{S}_1 (\hat{n} \cdot \vec{v}_1)^3 - \frac{16}{3} \vec{S}_1 \cdot \vec{S}_1 (\hat{n} \cdot \vec{v}_1)^3 - 30\hat{n} \cdot \vec{a}_1 (\hat{n} \cdot \vec{S}_1)^2 (\hat{n} \cdot \vec{v}_1)^2 + 5\hat{n} \cdot \vec{a}_2 (\hat{n} \cdot \vec{S}_1)^2 (\hat{n} \cdot \vec{v}_1)^2 - \right. \\ & 2\hat{n} \cdot \vec{S}_1 \hat{n} \cdot \vec{S}_1 \hat{n} \cdot \vec{v}_2 (\hat{n} \cdot \vec{v}_1)^2 - 2\hat{n} \cdot \vec{S}_1 \vec{S}_1 \cdot \vec{v}_1 (\hat{n} \cdot \vec{v}_1)^2 + \frac{1}{3} \hat{n} \cdot \vec{S}_1 \vec{S}_1 \cdot \vec{v}_2 (\hat{n} \cdot \vec{v}_1)^2 + \\ & \frac{4}{3} \hat{n} \cdot \vec{v}_2 \vec{S}_1 \cdot \vec{S}_1 (\hat{n} \cdot \vec{v}_1)^2 + 9\hat{n} \cdot \vec{S}_1 \vec{S}_1 \cdot \vec{a}_1 (\hat{n} \cdot \vec{v}_1)^2 - \frac{5}{3} \hat{n} \cdot \vec{S}_1 \vec{S}_1 \cdot \vec{a}_2 (\hat{n} \cdot \vec{v}_1)^2 + 2\hat{n} \cdot \vec{a}_1 \vec{S}_1 \cdot \vec{S}_1 (\hat{n} \cdot \vec{v}_1)^2 - \\ & \frac{4}{3} \hat{n} \cdot \vec{a}_2 \vec{S}_1 \cdot \vec{S}_1 (\hat{n} \cdot \vec{v}_1)^2 - 2\hat{n} \cdot \vec{S}_1 \vec{S}_1 \cdot \vec{v}_1 (\hat{n} \cdot \vec{v}_1)^2 + \frac{1}{3} \hat{n} \cdot \vec{S}_1 \vec{S}_1 \cdot \vec{v}_2 (\hat{n} \cdot \vec{v}_1)^2 - 5\hat{n} \cdot \vec{a}_1 (\hat{n} \cdot \vec{S}_1)^2 \hat{n} \cdot \vec{v}_2 \hat{n} \cdot \vec{v}_1 - \\ & \frac{4}{3} \hat{n} \cdot \vec{S}_1 \hat{n} \cdot \vec{v}_2 \vec{S}_1 \cdot \vec{v}_1 \hat{n} \cdot \vec{v}_1 + \frac{5}{6} (\hat{n} \cdot \vec{S}_1)^2 \vec{a}_1 \cdot \vec{v}_2 \hat{n} \cdot \vec{v}_1 - \frac{10}{3} \hat{n} \cdot \vec{S}_1 \hat{n} \cdot \vec{v}_2 \vec{S}_1 \cdot \vec{a}_1 \hat{n} \cdot \vec{v}_1 + \\ & \frac{4}{3} \hat{n} \cdot \vec{a}_1 \hat{n} \cdot \vec{v}_2 \vec{S}_1 \cdot \vec{S}_1 \hat{n} \cdot \vec{v}_1 - \frac{1}{3} \vec{a}_1 \cdot \vec{v}_2 \vec{S}_1 \cdot \vec{S}_1 \hat{n} \cdot \vec{v}_1 + 15\hat{n} \cdot \vec{a}_1 \hat{n} \cdot \vec{S}_1 \vec{S}_1 \cdot \vec{v}_1 \hat{n} \cdot \vec{v}_1 + \\ & \frac{2}{3} \hat{n} \cdot \vec{a}_2 \hat{n} \cdot \vec{S}_1 \vec{S}_1 \cdot \vec{v}_1 \hat{n} \cdot \vec{v}_1 - \frac{4}{3} \hat{n} \cdot \vec{S}_1 \hat{n} \cdot \vec{v}_2 \vec{S}_1 \cdot \vec{v}_1 \hat{n} \cdot \vec{v}_1 - 2\vec{S}_1 \cdot \vec{v}_1 \vec{S}_1 \cdot \vec{v}_1 \hat{n} \cdot \vec{v}_1 + \frac{1}{3} \vec{S}_1 \cdot \vec{v}_2 \vec{S}_1 \cdot \vec{v}_1 \hat{n} \cdot \vec{v}_1 - \\ & 3\vec{S}_1 \cdot \vec{a}_1 \vec{S}_1 \cdot \vec{v}_1 \hat{n} \cdot \vec{v}_1 - \frac{1}{6} \vec{S}_1 \cdot \vec{a}_2 \vec{S}_1 \cdot \vec{v}_1 \hat{n} \cdot \vec{v}_1 + \frac{5}{3} \hat{n} \cdot \vec{a}_1 \hat{n} \cdot \vec{S}_1 \vec{S}_1 \cdot \vec{v}_2 \hat{n} \cdot \vec{v}_1 + \frac{1}{3} \vec{S}_1 \cdot \vec{v}_1 \vec{S}_1 \cdot \vec{v}_2 \hat{n} \cdot \vec{v}_1 + \\ & \frac{5}{6} \vec{S}_1 \cdot \vec{a}_1 \vec{S}_1 \cdot \vec{v}_2 \hat{n} \cdot \vec{v}_1 + \frac{25}{2} (\hat{n} \cdot \vec{S}_1)^2 \vec{v}_1 \cdot \vec{a}_1 \hat{n} \cdot \vec{v}_1 - \frac{3}{2} \vec{S}_1 \cdot \vec{S}_1 \vec{v}_1 \cdot \vec{a}_1 \hat{n} \cdot \vec{v}_1 - \frac{5}{3} (\hat{n} \cdot \vec{S}_1)^2 \vec{v}_1 \cdot \vec{a}_2 \hat{n} \cdot \vec{v}_1 + \\ & \frac{2}{3} \vec{S}_1 \cdot \vec{S}_1 \vec{v}_1 \cdot \vec{a}_2 \hat{n} \cdot \vec{v}_1 + 2\vec{S}_1 \cdot \vec{S}_1 \vec{v}_1 \cdot \vec{v}_1 \hat{n} \cdot \vec{v}_1 + \frac{2}{3} \hat{n} \cdot \vec{S}_1 \hat{n} \cdot \vec{S}_1 \vec{v}_1 \cdot \vec{v}_2 \hat{n} \cdot \vec{v}_1 - \frac{2}{3} \vec{S}_1 \cdot \vec{S}_1 \vec{v}_1 \cdot \vec{v}_2 \hat{n} \cdot \vec{v}_1 + \\ & 30\hat{n} \cdot \vec{a}_1 (\hat{n} \cdot \vec{S}_1)^2 (\hat{n} \cdot \vec{v}_2)^2 - \frac{3}{2} \hat{n} \cdot \vec{a}_1 (\vec{S}_1 \cdot \vec{v}_1)^2 - \frac{1}{3} \hat{n} \cdot \vec{a}_2 (\vec{S}_1 \cdot \vec{v}_1)^2 + \frac{5}{2} \hat{n} \cdot \vec{a}_1 (\vec{S}_1 \cdot \vec{v}_2)^2 - \\ & 10(\hat{n} \cdot \vec{S}_1)^2 \hat{n} \cdot \vec{v}_2 \vec{a}_1 \cdot \vec{v}_2 - 4\hat$$

$$\begin{aligned}
& \frac{1}{6} \hat{n} \cdot \vec{S}_1 \vec{S}_1 \cdot \vec{v}_1 \vec{v}_1 \cdot \vec{a}_2 + \frac{5}{2} \hat{n} \cdot \vec{a}_1 \left( \hat{n} \cdot \vec{S}_1 \right)^2 \vec{v}_1 \cdot \vec{v}_1 + \frac{5}{3} \hat{n} \cdot \vec{a}_2 \left( \hat{n} \cdot \vec{S}_1 \right)^2 \vec{v}_1 \cdot \vec{v}_1 + \frac{16}{3} \hat{n} \cdot \vec{S}_1 \hat{n} \cdot \vec{S}_1 \hat{n} \cdot \vec{v}_2 \vec{v}_1 \cdot \vec{v}_1 - \\
& 2 \hat{n} \cdot \vec{S}_1 \vec{S}_1 \cdot \vec{v}_1 \vec{v}_1 \cdot \vec{v}_1 - \frac{4}{3} \hat{n} \cdot \vec{S}_1 \vec{S}_1 \cdot \vec{v}_2 \vec{v}_1 \cdot \vec{v}_1 - \frac{4}{3} \hat{n} \cdot \vec{v}_2 \vec{S}_1 \cdot \vec{S}_1 \vec{v}_1 \cdot \vec{v}_1 - \hat{n} \cdot \vec{S}_1 \vec{S}_1 \cdot \vec{a}_1 \vec{v}_1 \cdot \vec{v}_1 - \\
& \frac{5}{6} \hat{n} \cdot \vec{S}_1 \vec{S}_1 \cdot \vec{a}_2 \vec{v}_1 \cdot \vec{v}_1 - \frac{1}{6} \hat{n} \cdot \vec{a}_2 \vec{S}_1 \cdot \vec{S}_1 \vec{v}_1 \cdot \vec{v}_1 - 2 \hat{n} \cdot \vec{S}_1 \vec{S}_1 \cdot \vec{v}_1 \vec{v}_1 \cdot \vec{v}_1 - \frac{4}{3} \hat{n} \cdot \vec{S}_1 \vec{S}_1 \cdot \vec{v}_2 \vec{v}_1 \cdot \vec{v}_1 + \\
& \frac{5}{6} \hat{n} \cdot \vec{a}_1 \left( \hat{n} \cdot \vec{S}_1 \right)^2 \vec{v}_1 \cdot \vec{v}_2 + \frac{1}{3} \hat{n} \cdot \vec{S}_1 \vec{S}_1 \cdot \vec{v}_1 \vec{v}_1 \cdot \vec{v}_2 + \frac{5}{6} \hat{n} \cdot \vec{S}_1 \vec{S}_1 \cdot \vec{a}_1 \vec{v}_1 \cdot \vec{v}_2 - \frac{1}{3} \hat{n} \cdot \vec{a}_1 \vec{S}_1 \cdot \vec{S}_1 \vec{v}_1 \cdot \vec{v}_2 + \\
& \frac{1}{3} \hat{n} \cdot \vec{S}_1 \vec{S}_1 \cdot \vec{v}_1 \vec{v}_1 \cdot \vec{v}_2 - 5 \hat{n} \cdot \vec{a}_1 \left( \hat{n} \cdot \vec{S}_1 \right)^2 \vec{v}_2 \cdot \vec{v}_2 + \hat{n} \cdot \vec{S}_1 \vec{S}_1 \cdot \vec{a}_1 \vec{v}_2 \cdot \vec{v}_2 + \frac{1}{2} \hat{n} \cdot \vec{a}_1 \vec{S}_1 \cdot \vec{S}_1 \vec{v}_2 \cdot \vec{v}_2 \Big) + \frac{1}{r^4} \\
& \left( -35 \left( \hat{n} \cdot \vec{S}_1 \right)^2 \left( \hat{n} \cdot \vec{v}_1 \right)^4 + \frac{25}{4} \vec{S}_1 \cdot \vec{S}_1 \left( \hat{n} \cdot \vec{v}_1 \right)^4 + 5 \left( \hat{n} \cdot \vec{S}_1 \right)^2 \hat{n} \cdot \vec{v}_2 \left( \hat{n} \cdot \vec{v}_1 \right)^3 - \frac{7}{4} \hat{n} \cdot \vec{v}_2 \vec{S}_1 \cdot \vec{S}_1 \left( \hat{n} \cdot \vec{v}_1 \right)^3 + \right. \\
& \frac{65}{4} \hat{n} \cdot \vec{S}_1 \vec{S}_1 \cdot \vec{v}_1 \left( \hat{n} \cdot \vec{v}_1 \right)^3 - \frac{5}{4} \hat{n} \cdot \vec{S}_1 \vec{S}_1 \cdot \vec{v}_2 \left( \hat{n} \cdot \vec{v}_1 \right)^3 + 40 \left( \hat{n} \cdot \vec{S}_1 \right)^2 \left( \hat{n} \cdot \vec{v}_2 \right)^2 \left( \hat{n} \cdot \vec{v}_1 \right)^2 - \\
& \frac{1}{4} \left( \vec{S}_1 \cdot \vec{v}_1 \right)^2 \left( \hat{n} \cdot \vec{v}_1 \right)^2 + \frac{5}{3} \left( \vec{S}_1 \cdot \vec{v}_2 \right)^2 \left( \hat{n} \cdot \vec{v}_1 \right)^2 - 8 \left( \hat{n} \cdot \vec{v}_2 \right)^2 \vec{S}_1 \cdot \vec{S}_1 \left( \hat{n} \cdot \vec{v}_1 \right)^2 + \\
& \frac{3}{2} \hat{n} \cdot \vec{S}_1 \hat{n} \cdot \vec{v}_2 \vec{S}_1 \cdot \vec{v}_1 \left( \hat{n} \cdot \vec{v}_1 \right)^2 - 20 \hat{n} \cdot \vec{S}_1 \hat{n} \cdot \vec{v}_2 \vec{S}_1 \cdot \vec{v}_2 \left( \hat{n} \cdot \vec{v}_1 \right)^2 - \frac{1}{4} \vec{S}_1 \cdot \vec{v}_1 \vec{S}_1 \cdot \vec{v}_2 \left( \hat{n} \cdot \vec{v}_1 \right)^2 + \\
& \frac{15}{8} \left( \hat{n} \cdot \vec{S}_1 \right)^2 \vec{v}_1 \cdot \vec{v}_1 \left( \hat{n} \cdot \vec{v}_1 \right)^2 - \frac{21}{8} \vec{S}_1 \cdot \vec{S}_1 \vec{v}_1 \cdot \vec{v}_1 \left( \hat{n} \cdot \vec{v}_1 \right)^2 - \frac{15}{8} \left( \hat{n} \cdot \vec{S}_1 \right)^2 \vec{v}_1 \cdot \vec{v}_2 \left( \hat{n} \cdot \vec{v}_1 \right)^2 + \\
& \frac{7}{8} \vec{S}_1 \cdot \vec{S}_1 \vec{v}_1 \cdot \vec{v}_2 \left( \hat{n} \cdot \vec{v}_1 \right)^2 - 5 \left( \hat{n} \cdot \vec{S}_1 \right)^2 \vec{v}_2 \cdot \vec{v}_2 \left( \hat{n} \cdot \vec{v}_1 \right)^2 + \frac{4}{3} \vec{S}_1 \cdot \vec{S}_1 \vec{v}_2 \cdot \vec{v}_2 \left( \hat{n} \cdot \vec{v}_1 \right)^2 - \hat{n} \cdot \vec{v}_2 \left( \vec{S}_1 \cdot \vec{v}_1 \right)^2 \hat{n} \cdot \vec{v}_1 + \\
& 4 \hat{n} \cdot \vec{S}_1 \left( \hat{n} \cdot \vec{v}_2 \right)^2 \vec{S}_1 \cdot \vec{v}_1 \hat{n} \cdot \vec{v}_1 - \frac{4}{3} \hat{n} \cdot \vec{v}_2 \vec{S}_1 \cdot \vec{v}_1 \vec{S}_1 \cdot \vec{v}_2 \hat{n} \cdot \vec{v}_1 - \frac{45}{4} \left( \hat{n} \cdot \vec{S}_1 \right)^2 \hat{n} \cdot \vec{v}_2 \vec{v}_1 \cdot \vec{v}_1 \hat{n} \cdot \vec{v}_1 + \\
& \frac{5}{2} \hat{n} \cdot \vec{v}_2 \vec{S}_1 \cdot \vec{S}_1 \vec{v}_1 \cdot \vec{v}_1 \hat{n} \cdot \vec{v}_1 + \frac{25}{4} \hat{n} \cdot \vec{S}_1 \vec{S}_1 \cdot \vec{v}_1 \vec{v}_1 \cdot \vec{v}_1 \hat{n} \cdot \vec{v}_1 + \frac{15}{4} \hat{n} \cdot \vec{S}_1 \vec{S}_1 \cdot \vec{v}_2 \vec{v}_1 \cdot \vec{v}_1 \hat{n} \cdot \vec{v}_1 - \\
& 20 \left( \hat{n} \cdot \vec{S}_1 \right)^2 \hat{n} \cdot \vec{v}_2 \vec{v}_1 \cdot \vec{v}_2 \hat{n} \cdot \vec{v}_1 + \frac{16}{3} \hat{n} \cdot \vec{v}_2 \vec{S}_1 \cdot \vec{S}_1 \vec{v}_1 \cdot \vec{v}_2 \hat{n} \cdot \vec{v}_1 - \frac{1}{2} \hat{n} \cdot \vec{S}_1 \vec{S}_1 \cdot \vec{v}_1 \vec{v}_1 \cdot \vec{v}_2 \hat{n} \cdot \vec{v}_1 + \\
& \frac{20}{3} \hat{n} \cdot \vec{S}_1 \vec{S}_1 \cdot \vec{v}_2 \vec{v}_1 \cdot \vec{v}_2 \hat{n} \cdot \vec{v}_1 - \frac{2}{3} \hat{n} \cdot \vec{S}_1 \vec{S}_1 \cdot \vec{v}_1 \vec{v}_2 \cdot \vec{v}_2 \hat{n} \cdot \vec{v}_1 - \frac{4}{3} \left( \hat{n} \cdot \vec{v}_2 \right)^2 \left( \vec{S}_1 \cdot \vec{v}_1 \right)^2 + \\
& \frac{15}{8} \left( \hat{n} \cdot \vec{S}_1 \right)^2 \left( \vec{v}_1 \cdot \vec{v}_1 \right)^2 - \frac{1}{8} \vec{S}_1 \cdot \vec{S}_1 \left( \vec{v}_1 \cdot \vec{v}_1 \right)^2 + \frac{5}{3} \left( \hat{n} \cdot \vec{S}_1 \right)^2 \left( \vec{v}_1 \cdot \vec{v}_2 \right)^2 - \frac{2}{3} \vec{S}_1 \cdot \vec{S}_1 \left( \vec{v}_1 \cdot \vec{v}_2 \right)^2 + \\
& 10 \left( \hat{n} \cdot \vec{S}_1 \right)^2 \left( \hat{n} \cdot \vec{v}_2 \right)^2 \vec{v}_1 \cdot \vec{v}_1 - \frac{3}{2} \left( \vec{S}_1 \cdot \vec{v}_1 \right)^2 \vec{v}_1 \cdot \vec{v}_1 + \frac{5}{6} \left( \vec{S}_1 \cdot \vec{v}_2 \right)^2 \vec{v}_1 \cdot \vec{v}_1 - \frac{2}{3} \left( \hat{n} \cdot \vec{v}_2 \right)^2 \vec{S}_1 \cdot \vec{S}_1 \vec{v}_1 \cdot \vec{v}_1 + \\
& \hat{n} \cdot \vec{S}_1 \hat{n} \cdot \vec{v}_2 \vec{S}_1 \cdot \vec{v}_1 \vec{v}_1 \cdot \vec{v}_1 - \frac{20}{3} \hat{n} \cdot \vec{S}_1 \hat{n} \cdot \vec{v}_2 \vec{S}_1 \cdot \vec{v}_2 \vec{v}_1 \cdot \vec{v}_1 - \frac{1}{4} \vec{S}_1 \cdot \vec{v}_1 \vec{S}_1 \cdot \vec{v}_2 \vec{v}_1 \cdot \vec{v}_1 + \frac{1}{4} \left( \vec{S}_1 \cdot \vec{v}_1 \right)^2 \vec{v}_1 \cdot \vec{v}_2 - \\
& \frac{4}{3} \hat{n} \cdot \vec{S}_1 \hat{n} \cdot \vec{v}_2 \vec{S}_1 \cdot \vec{v}_1 \vec{v}_1 \cdot \vec{v}_2 + \frac{1}{3} \vec{S}_1 \cdot \vec{v}_1 \vec{S}_1 \cdot \vec{v}_2 \vec{v}_1 \cdot \vec{v}_2 + \frac{15}{8} \left( \hat{n} \cdot \vec{S}_1 \right)^2 \vec{v}_1 \cdot \vec{v}_1 \vec{v}_1 \cdot \vec{v}_2 - \frac{5}{8} \vec{S}_1 \cdot \vec{S}_1 \vec{v}_1 \cdot \vec{v}_1 \vec{v}_1 \cdot \vec{v}_2 + \\
& \left. \frac{1}{3} \left( \vec{S}_1 \cdot \vec{v}_1 \right)^2 \vec{v}_2 \cdot \vec{v}_2 - \frac{5}{3} \left( \hat{n} \cdot \vec{S}_1 \right)^2 \vec{v}_1 \cdot \vec{v}_1 \vec{v}_2 \cdot \vec{v}_2 + \frac{1}{6} \vec{S}_1 \cdot \vec{S}_1 \vec{v}_1 \cdot \vec{v}_1 \vec{v}_2 \cdot \vec{v}_2 \right) \Bigg\} m_2 C_{ES^2_1} \Bigg\}
\end{aligned}$$

{DiagS1CES2[2, 2, 49],

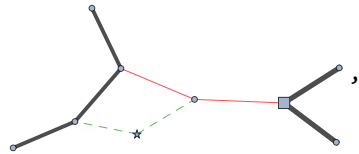

$$\begin{aligned}
& \frac{1}{m_1} G^2 \left( \frac{1}{r} \left( -\frac{4}{3} \hat{n} \cdot \vec{a}_2 \left( \hat{n} \cdot \vec{S}_1 \right)^2 + \frac{4}{3} \vec{S}_1 \cdot \vec{a}_2 \hat{n} \cdot \vec{S}_1 - \frac{4}{3} \hat{n} \cdot \vec{S}_1 \hat{n} \cdot \vec{a}_2 \hat{n} \cdot \vec{S}_1 - \right. \right. \\
& \left. \left. \frac{4}{3} \hat{n} \cdot \vec{a}_2 \vec{S}_1 \cdot \vec{S}_1 + \frac{2}{3} \hat{n} \cdot \vec{S}_1 \vec{S}_1 \cdot \vec{a}_2 - \frac{4}{3} \hat{n} \cdot \vec{a}_2 \vec{S}_1 \cdot \vec{S}_1 + \frac{2}{3} \hat{n} \cdot \vec{S}_1 \vec{S}_1 \cdot \vec{a}_2 \right) + \frac{1}{r^2} \right.
\end{aligned}$$

[illegible]

$$\begin{aligned} & \frac{8}{3} (\hat{n} \cdot \vec{S}_1)^2 \hat{n} \cdot \vec{v}_1 \vec{v}_2 \cdot \vec{a}_2 - \frac{2}{3} \hat{n} \cdot \vec{v}_1 \vec{S}_1 \cdot \vec{S}_1 \vec{v}_2 \cdot \vec{a}_2 - \frac{4}{3} \hat{n} \cdot \vec{S}_1 \vec{S}_1 \cdot \vec{v}_1 \vec{v}_2 \cdot \vec{a}_2 + \frac{14}{3} \hat{n} \cdot \vec{S}_1 \vec{S}_1 \cdot \vec{v}_2 \vec{v}_2 \cdot \vec{a}_2 - \\ & \frac{8}{3} \hat{n} \cdot \vec{a}_1 (\hat{n} \cdot \vec{S}_1)^2 \vec{v}_2 \cdot \vec{v}_2 + \frac{4}{3} \hat{n} \cdot \vec{a}_2 (\hat{n} \cdot \vec{S}_1)^2 \vec{v}_2 \cdot \vec{v}_2 - \frac{32}{3} \hat{n} \cdot \vec{S}_1 \hat{n} \cdot \vec{S}_1 \hat{n} \cdot \vec{v}_1 \vec{v}_2 \cdot \vec{v}_2 + \frac{8}{3} \hat{n} \cdot \vec{S}_1 \vec{S}_1^{\frac{1}{2}} \cdot \vec{v}_1 \vec{v}_2 \cdot \vec{v}_2 - \\ & \hat{n} \cdot \vec{S}_1 \vec{S}_1^{\frac{1}{2}} \cdot \vec{v}_2 \vec{v}_2 \cdot \vec{v}_2 + \frac{8}{3} \hat{n} \cdot \vec{v}_1 \vec{S}_1 \cdot \vec{S}_1 \vec{v}_2 \cdot \vec{v}_2 + \frac{4}{3} \hat{n} \cdot \vec{S}_1 \vec{S}_1 \cdot \vec{a}_1 \vec{v}_2 \cdot \vec{v}_2 - \frac{2}{3} \hat{n} \cdot \vec{S}_1 \vec{S}_1 \cdot \vec{a}_2 \vec{v}_2 \cdot \vec{v}_2 + \\ & \left. \frac{2}{3} \hat{n} \cdot \vec{a}_1 \vec{S}_1 \cdot \vec{S}_1 \vec{v}_2 \cdot \vec{v}_2 - \frac{4}{3} \hat{n} \cdot \vec{a}_2 \vec{S}_1 \cdot \vec{S}_1 \vec{v}_2 \cdot \vec{v}_2 + \frac{8}{3} \hat{n} \cdot \vec{S}_1 \vec{S}_1 \cdot \vec{v}_1 \vec{v}_2 \cdot \vec{v}_2 - \hat{n} \cdot \vec{S}_1 \vec{S}_1 \cdot \vec{v}_2 \vec{v}_2 \cdot \vec{v}_2 \right) + \frac{1}{r^4} \\ & \left( -48 (\hat{n} \cdot \vec{S}_1)^2 (\hat{n} \cdot \vec{v}_2)^4 - 12 \vec{S}_1 \cdot \vec{S}_1 (\hat{n} \cdot \vec{v}_2)^4 + 16 (\hat{n} \cdot \vec{S}_1)^2 \hat{n} \cdot \vec{v}_1 (\hat{n} \cdot \vec{v}_2)^3 + 4 \hat{n} \cdot \vec{v}_1 \vec{S}_1 \cdot \vec{S}_1 (\hat{n} \cdot \vec{v}_2)^3 - \right. \\ & 4 \hat{n} \cdot \vec{S}_1 \vec{S}_1 \cdot \vec{v}_1 (\hat{n} \cdot \vec{v}_2)^3 + 48 \hat{n} \cdot \vec{S}_1 \vec{S}_1 \cdot \vec{v}_2 (\hat{n} \cdot \vec{v}_2)^3 + 64 (\hat{n} \cdot \vec{S}_1)^2 (\hat{n} \cdot \vec{v}_1)^2 (\hat{n} \cdot \vec{v}_2)^2 + \frac{8}{3} (\vec{S}_1 \cdot \vec{v}_1)^2 (\hat{n} \cdot \vec{v}_2)^2 - \\ & 12 (\vec{S}_1 \cdot \vec{v}_2)^2 (\hat{n} \cdot \vec{v}_2)^2 + 16 (\hat{n} \cdot \vec{v}_1)^2 \vec{S}_1 \cdot \vec{S}_1 (\hat{n} \cdot \vec{v}_2)^2 - 32 \hat{n} \cdot \vec{S}_1 \hat{n} \cdot \vec{v}_1 \vec{S}_1 \cdot \vec{v}_1 (\hat{n} \cdot \vec{v}_2)^2 - \\ & 12 \hat{n} \cdot \vec{S}_1 \hat{n} \cdot \vec{v}_1 \vec{S}_1 \cdot \vec{v}_2 (\hat{n} \cdot \vec{v}_2)^2 + 2 \vec{S}_1 \cdot \vec{v}_1 \vec{S}_1 \cdot \vec{v}_2 (\hat{n} \cdot \vec{v}_2)^2 - 8 (\hat{n} \cdot \vec{S}_1)^2 \vec{v}_1 \cdot \vec{v}_1 (\hat{n} \cdot \vec{v}_2)^2 - \\ & \frac{8}{3} \vec{S}_1 \cdot \vec{S}_1 \vec{v}_1 \cdot \vec{v}_1 (\hat{n} \cdot \vec{v}_2)^2 - 6 (\hat{n} \cdot \vec{S}_1)^2 \vec{v}_1 \cdot \vec{v}_2 (\hat{n} \cdot \vec{v}_2)^2 - 2 \vec{S}_1 \cdot \vec{S}_1 \vec{v}_1 \cdot \vec{v}_2 (\hat{n} \cdot \vec{v}_2)^2 + \\ & 6 (\hat{n} \cdot \vec{S}_1)^2 \vec{v}_2 \cdot \vec{v}_2 (\hat{n} \cdot \vec{v}_2)^2 + 12 \vec{S}_1 \cdot \vec{S}_1 \vec{v}_2 \cdot \vec{v}_2 (\hat{n} \cdot \vec{v}_2)^2 + 2 \hat{n} \cdot \vec{v}_1 (\vec{S}_1 \cdot \vec{v}_2)^2 \hat{n} \cdot \vec{v}_2 - \\ & 32 \hat{n} \cdot \vec{S}_1 (\hat{n} \cdot \vec{v}_1)^2 \vec{S}_1 \cdot \vec{v}_2 \hat{n} \cdot \vec{v}_2 + \frac{32}{3} \hat{n} \cdot \vec{v}_1 \vec{S}_1 \cdot \vec{v}_1 \vec{S}_1 \cdot \vec{v}_2 \hat{n} \cdot \vec{v}_2 + \frac{16}{3} \hat{n} \cdot \vec{S}_1 \vec{S}_1 \cdot \vec{v}_2 \vec{v}_1 \cdot \vec{v}_1 \hat{n} \cdot \vec{v}_2 - \\ & 32 (\hat{n} \cdot \vec{S}_1)^2 \hat{n} \cdot \vec{v}_1 \vec{v}_1 \cdot \vec{v}_2 \hat{n} \cdot \vec{v}_2 - \frac{32}{3} \hat{n} \cdot \vec{v}_1 \vec{S}_1 \cdot \vec{S}_1 \vec{v}_1 \cdot \vec{v}_2 \hat{n} \cdot \vec{v}_2 + \frac{32}{3} \hat{n} \cdot \vec{S}_1 \vec{S}_1 \cdot \vec{v}_1 \vec{v}_1 \cdot \vec{v}_2 \hat{n} \cdot \vec{v}_2 + \\ & 4 \hat{n} \cdot \vec{S}_1 \vec{S}_1 \cdot \vec{v}_2 \vec{v}_1 \cdot \vec{v}_2 \hat{n} \cdot \vec{v}_2 - 12 (\hat{n} \cdot \vec{S}_1)^2 \hat{n} \cdot \vec{v}_1 \vec{v}_2 \cdot \vec{v}_2 \hat{n} \cdot \vec{v}_2 - 2 \hat{n} \cdot \vec{v}_1 \vec{S}_1 \cdot \vec{S}_1 \vec{v}_2 \cdot \vec{v}_2 \hat{n} \cdot \vec{v}_2 + \\ & 4 \hat{n} \cdot \vec{S}_1 \vec{S}_1 \cdot \vec{v}_1 \vec{v}_2 \cdot \vec{v}_2 \hat{n} \cdot \vec{v}_2 - 4 \hat{n} \cdot \vec{S}_1 \vec{S}_1 \cdot \vec{v}_2 \vec{v}_2 \cdot \vec{v}_2 \hat{n} \cdot \vec{v}_2 + \frac{8}{3} (\hat{n} \cdot \vec{v}_1)^2 (\vec{S}_1 \cdot \vec{v}_2)^2 + \\ & \frac{8}{3} (\hat{n} \cdot \vec{S}_1)^2 (\vec{v}_1 \cdot \vec{v}_2)^2 + \frac{4}{3} \vec{S}_1 \cdot \vec{S}_1 (\vec{v}_1 \cdot \vec{v}_2)^2 + 2 (\hat{n} \cdot \vec{S}_1)^2 (\vec{v}_2 \cdot \vec{v}_2)^2 - \frac{3}{2} \vec{S}_1 \cdot \vec{S}_1 (\vec{v}_2 \cdot \vec{v}_2)^2 - \\ & \frac{2}{3} (\vec{S}_1 \cdot \vec{v}_2)^2 \vec{v}_1 \cdot \vec{v}_1 - \frac{1}{2} (\vec{S}_1 \cdot \vec{v}_2)^2 \vec{v}_1 \cdot \vec{v}_2 + \frac{32}{3} \hat{n} \cdot \vec{S}_1 \hat{n} \cdot \vec{v}_1 \vec{S}_1 \cdot \vec{v}_2 \vec{v}_1 \cdot \vec{v}_2 - \frac{8}{3} \vec{S}_1 \cdot \vec{v}_1 \vec{S}_1 \cdot \vec{v}_2 \vec{v}_1 \cdot \vec{v}_2 + \\ & 16 (\hat{n} \cdot \vec{S}_1)^2 (\hat{n} \cdot \vec{v}_1)^2 \vec{v}_2 \cdot \vec{v}_2 + \frac{4}{3} (\vec{S}_1 \cdot \vec{v}_1)^2 \vec{v}_2 \cdot \vec{v}_2 + \frac{1}{2} (\vec{S}_1 \cdot \vec{v}_2)^2 \vec{v}_2 \cdot \vec{v}_2 - \frac{8}{3} (\hat{n} \cdot \vec{v}_1)^2 \vec{S}_1 \cdot \vec{S}_1 \vec{v}_2 \cdot \vec{v}_2 - \\ & \left. \frac{32}{3} \hat{n} \cdot \vec{S}_1 \hat{n} \cdot \vec{v}_1 \vec{S}_1 \cdot \vec{v}_1 \vec{v}_2 \cdot \vec{v}_2 + 4 \hat{n} \cdot \vec{S}_1 \hat{n} \cdot \vec{v}_1 \vec{S}_1 \cdot \vec{v}_2 \vec{v}_2 \cdot \vec{v}_2 - \vec{S}_1 \cdot \vec{v}_1 \vec{S}_1 \cdot \vec{v}_2 \vec{v}_2 \cdot \vec{v}_2 - \frac{8}{3} (\hat{n} \cdot \vec{S}_1)^2 \vec{v}_1 \cdot \vec{v}_1 \vec{v}_2 \cdot \vec{v}_2 + \right. \\ & \left. \frac{2}{3} \vec{S}_1 \cdot \vec{S}_1 \vec{v}_1 \cdot \vec{v}_1 \vec{v}_2 \cdot \vec{v}_2 + 2 (\hat{n} \cdot \vec{S}_1)^2 \vec{v}_1 \cdot \vec{v}_2 \vec{v}_2 \cdot \vec{v}_2 + \frac{1}{2} \vec{S}_1 \cdot \vec{S}_1 \vec{v}_1 \cdot \vec{v}_2 \vec{v}_2 \cdot \vec{v}_2 \right) m_{\text{ES}}^2 C_{\text{ES}^2} \} \end{aligned}$$

$$\{\text{DiagS1CES2}[2, 2, 50],$$

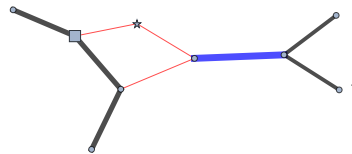

$$G^2 \left( \frac{1}{r^2} \left( -\frac{2}{3} \hat{n} \cdot \vec{S_1} \hat{n} \cdot \vec{a_2} \hat{n} \cdot \vec{S_1} \hat{n} \cdot \vec{v_2} + \frac{1}{6} \hat{n} \cdot \vec{S_1} \vec{S_1} \cdot \vec{a_2} \hat{n} \cdot \vec{v_2} - \frac{4}{3} \hat{n} \cdot \vec{a_2} \vec{S_1} \cdot \vec{S_1} \hat{n} \cdot \vec{v_2} + \frac{1}{6} \hat{n} \cdot \vec{S_1} \vec{S_1} \cdot \vec{a_2} \hat{n} \cdot \vec{v_2} + \frac{1}{6} \hat{n} \cdot \vec{a_2} \hat{n} \cdot \vec{S_1} \vec{S_1} \cdot \vec{v_2} - \frac{1}{3} \vec{S_1} \cdot \vec{v_2} \vec{S_1} \cdot \vec{a_2} + \frac{1}{6} \hat{n} \cdot \vec{S_1} \hat{n} \cdot \vec{a_2} \vec{S_1} \cdot \vec{v_2} - \frac{1}{3} \vec{S_1} \cdot \vec{a_2} \vec{S_1} \cdot \vec{v_2} - \frac{1}{3} \hat{n} \cdot \vec{S_1} \hat{n} \cdot \vec{S_1} \vec{v_2} \cdot \vec{a_2} + \frac{5}{3} \vec{S_1} \cdot \vec{S_1} \vec{v_2} \cdot \vec{a_2} \right) + \frac{1}{r^3} \right. \\ \left. \left( -2 \hat{n} \cdot \vec{S_1} \hat{n} \cdot \vec{S_1} (\hat{n} \cdot \vec{v_2})^3 - \frac{8}{3} \vec{S_1} \cdot \vec{S_1} (\hat{n} \cdot \vec{v_2})^3 + \frac{3}{4} \hat{n} \cdot \vec{S_1} \hat{n} \cdot \vec{S_1} \hat{n} \cdot \vec{v_1} (\hat{n} \cdot \vec{v_2})^2 + \frac{1}{4} \hat{n} \cdot \vec{S_1} \vec{S_1} \cdot \vec{v_1} (\hat{n} \cdot \vec{v_2})^2 + \right. \right. \\ \left. \left. \hat{n} \cdot \vec{S_1} \vec{S_1} \cdot \vec{v_2} (\hat{n} \cdot \vec{v_2})^2 + \frac{5}{4} \hat{n} \cdot \vec{v_1} \vec{S_1} \cdot \vec{S_1} (\hat{n} \cdot \vec{v_2})^2 + \frac{1}{4} \hat{n} \cdot \vec{S_1} \vec{S_1} \cdot \vec{v_1} (\hat{n} \cdot \vec{v_2})^2 + \hat{n} \cdot \vec{S_1} \vec{S_1} \cdot \vec{v_2} (\hat{n} \cdot \vec{v_2})^2 + \frac{5}{4} \hat{n} \cdot \vec{a_2} \right. \right. \\ \left. \left. (\hat{n} \cdot \vec{S_1})^2 \hat{n} \cdot \vec{v_1} \hat{n} \cdot \vec{v_2} - \frac{1}{2} \hat{n} \cdot \vec{S_1} \hat{n} \cdot \vec{v_1} \vec{S_1} \cdot \vec{v_2} \hat{n} \cdot \vec{v_2} - \frac{1}{6} \hat{n} \cdot \vec{S_1} \hat{n} \cdot \vec{v_1} \vec{S_1} \cdot \vec{a_2} \hat{n} \cdot \vec{v_2} + \frac{17}{12} \hat{n} \cdot \vec{a_2} \hat{n} \cdot \vec{v_1} \vec{S_1} \cdot \vec{S_1} \hat{n} \cdot \vec{v_2} - \right. \right. \\ \left. \left. \frac{7}{6} \hat{n} \cdot \vec{a_2} \hat{n} \cdot \vec{S_1} \vec{S_1} \cdot \vec{v_1} \hat{n} \cdot \vec{v_2} + \frac{1}{6} \vec{S_1} \cdot \vec{a_2} \vec{S_1} \cdot \vec{v_1} \hat{n} \cdot \vec{v_2} - \frac{1}{2} \hat{n} \cdot \vec{S_1} \hat{n} \cdot \vec{v_1} \vec{S_1} \cdot \vec{v_2} \hat{n} \cdot \vec{v_2} - \frac{1}{\vec{S_1} \cdot \vec{v_2} \vec{S_1} \cdot \vec{v_2}} \hat{n} \cdot \vec{v_2} - \right. \right. \\ \left. \left. \frac{1}{2} \hat{n} \cdot \vec{S_1} \hat{n} \cdot \vec{S_1} \vec{v_2} \cdot \vec{a_2} + \frac{1}{6} \hat{n} \cdot \vec{S_1} \vec{S_1} \cdot \vec{v_2} \cdot \vec{a_2} + \frac{1}{6} \hat{n} \cdot \vec{a_2} \hat{n} \cdot \vec{S_1} \vec{S_1} \cdot \vec{v_2} + \frac{1}{6} \hat{n} \cdot \vec{S_1} \vec{S_1} \cdot \vec{a_2} \hat{n} \cdot \vec{v_2} + \frac{1}{6} \hat{n} \cdot \vec{a_2} \hat{n} \cdot \vec{S_1} \vec{S_1} \cdot \vec{v_2} \right) \right)$$

gS1CES2[2, 2, 51],

$$G^2 \left( \frac{1}{r} \left( 4 \hat{n} \cdot \vec{\bar{S}}_1 \hat{n} \cdot \vec{\bar{S}}_1 \hat{n} \cdot \vec{\bar{v}}_2 + \frac{4}{3} \hat{n} \cdot \vec{\bar{S}}_1 \hat{n} \cdot \vec{\bar{S}}_1 \hat{n} \cdot \vec{\bar{v}}_2 + 4 \vec{\bar{S}}_1 \cdot \vec{\bar{S}}_1 \hat{n} \cdot \vec{\bar{v}}_2 + \right. \right.$$
  

$$\left. \frac{4}{3} \vec{\bar{S}}_1 \cdot \vec{\bar{S}}_1 \hat{n} \cdot \vec{\bar{v}}_2 - 2 \hat{n} \cdot \vec{\bar{S}}_1 \vec{\bar{S}}_1 \cdot \vec{\bar{v}}_2 - 2 \hat{n} \cdot \vec{\bar{S}}_1 \vec{\bar{S}}_1 \cdot \vec{\bar{v}}_2 - \frac{2}{3} \hat{n} \cdot \vec{\bar{S}}_1 \vec{\bar{S}}_1 \cdot \vec{\bar{v}}_2 - \frac{2}{3} \hat{n} \cdot \vec{\bar{S}}_1 \vec{\bar{S}}_1 \cdot \vec{\bar{v}}_2 \right) + \frac{1}{r^2}$$
  

$$\left( -8 \hat{n} \cdot \vec{\bar{v}}_1 \hat{n} \cdot \vec{\bar{v}}_2 \left( \hat{n} \cdot \vec{\bar{S}}_1 \right)^2 + 2 \vec{\bar{v}}_1 \cdot \vec{\bar{v}}_2 \left( \hat{n} \cdot \vec{\bar{S}}_1 \right)^2 - 4 \hat{n} \cdot \vec{\bar{a}}_1 \hat{n} \cdot \vec{\bar{S}}_1 \hat{n} \cdot \vec{\bar{v}}_2 \hat{n} \cdot \vec{\bar{S}}_1 + 5 \hat{n} \cdot \vec{\bar{v}}_2 \vec{\bar{S}}_1 \cdot \vec{\bar{v}}_1 \hat{n} \cdot \vec{\bar{S}}_1 + \right.$$
  

$$4 \hat{n} \cdot \vec{\bar{v}}_1 \vec{\bar{S}}_1 \cdot \vec{\bar{v}}_2 \hat{n} \cdot \vec{\bar{S}}_1 + \hat{n} \cdot \vec{\bar{S}}_1 \vec{\bar{a}}_1 \cdot \vec{\bar{v}}_2 \hat{n} \cdot \vec{\bar{S}}_1 + \frac{3}{2} \hat{n} \cdot \vec{\bar{v}}_2 \vec{\bar{S}}_1 \cdot \vec{\bar{a}}_1 \hat{n} \cdot \vec{\bar{S}}_1 + \hat{n} \cdot \vec{\bar{a}}_1 \vec{\bar{S}}_1 \cdot \vec{\bar{v}}_2 \hat{n} \cdot \vec{\bar{S}}_1 - \frac{2}{3} \hat{n} \cdot \vec{\bar{a}}_1 \left( \hat{n} \cdot \vec{\bar{S}}_1 \right)^2 \hat{n} \cdot \vec{\bar{v}}_2 -$$
  

$$8 \hat{n} \cdot \vec{\bar{S}}_1 \hat{n} \cdot \vec{\bar{S}}_1 \hat{n} \cdot \vec{\bar{v}}_1 \hat{n} \cdot \vec{\bar{v}}_2 + \frac{1}{6} \left( \hat{n} \cdot \vec{\bar{S}}_1 \right)^2 \vec{\bar{a}}_1 \cdot \vec{\bar{v}}_2 - 7 \hat{n} \cdot \vec{\bar{v}}_1 \hat{n} \cdot \vec{\bar{v}}_2 \vec{\bar{S}}_1 \cdot \vec{\bar{S}}_1 + \frac{3}{2} \hat{n} \cdot \vec{\bar{S}}_1 \hat{n} \cdot \vec{\bar{v}}_2 \vec{\bar{S}}_1 \cdot \vec{\bar{a}}_1 +$$
  

$$\hat{n} \cdot \vec{\bar{a}}_1 \hat{n} \cdot \vec{\bar{S}}_1 \vec{\bar{S}}_1 \cdot \vec{\bar{v}}_2 - \frac{5}{2} \vec{\bar{S}}_1 \cdot \vec{\bar{v}}_1 \vec{\bar{S}}_1 \cdot \vec{\bar{v}}_2 + \frac{5}{2} \hat{n} \cdot \vec{\bar{S}}_1 \hat{n} \cdot \vec{\bar{v}}_2 \vec{\bar{S}}_1 \cdot \vec{\bar{v}}_1 + 2 \hat{n} \cdot \vec{\bar{S}}_1 \hat{n} \cdot \vec{\bar{v}}_1 \vec{\bar{S}}_1 \cdot \vec{\bar{v}}_2 + \frac{1}{3} \hat{n} \cdot \vec{\bar{S}}_1 \hat{n} \cdot \vec{\bar{v}}_2 \vec{\bar{S}}_1 \cdot \vec{\bar{a}}_1 -$$
  

$$7 \hat{n} \cdot \vec{\bar{a}}_1 \hat{n} \cdot \vec{\bar{v}}_2 \vec{\bar{S}}_1 \cdot \vec{\bar{S}}_1 + \frac{7}{2} \vec{\bar{a}}_1 \cdot \vec{\bar{v}}_2 \vec{\bar{S}}_1 \cdot \vec{\bar{S}}_1 - 7 \hat{n} \cdot \vec{\bar{v}}_1 \hat{n} \cdot \vec{\bar{v}}_2 \vec{\bar{S}}_1 \cdot \vec{\bar{S}}_1 - \frac{3}{4} \vec{\bar{S}}_1 \cdot \vec{\bar{v}}_2 \vec{\bar{S}}_1 \cdot \vec{\bar{a}}_1 - \frac{4}{3} \hat{n} \cdot \vec{\bar{a}}_1 \hat{n} \cdot \vec{\bar{v}}_2 \vec{\bar{S}}_1 \cdot \vec{\bar{S}}_1 +$$
  

$$\frac{2}{3} \vec{\bar{a}}_1 \cdot \vec{\bar{v}}_2 \vec{\bar{S}}_1 \cdot \vec{\bar{S}}_1 + \frac{5}{2} \hat{n} \cdot \vec{\bar{S}}_1 \hat{n} \cdot \vec{\bar{v}}_2 \vec{\bar{S}}_1 \cdot \vec{\bar{v}}_1 - \frac{5}{4} \vec{\bar{S}}_1 \cdot \vec{\bar{v}}_2 \vec{\bar{S}}_1 \cdot \vec{\bar{v}}_1 + \frac{1}{3} \hat{n} \cdot \vec{\bar{a}}_1 \hat{n} \cdot \vec{\bar{S}}_1 \vec{\bar{S}}_1 \cdot \vec{\bar{v}}_2 + 2 \hat{n} \cdot \vec{\bar{S}}_1 \hat{n} \cdot \vec{\bar{v}}_1 \vec{\bar{S}}_1 \cdot \vec{\bar{v}}_2 -$$

$$\begin{aligned}
& \frac{3}{4} \vec{S}_1 \cdot \vec{a}_1 \vec{S}_1 \cdot \vec{v}_2 - \frac{5}{4} \vec{S}_1 \cdot \vec{v}_1 \vec{S}_1 \cdot \vec{v}_2 - \frac{1}{6} \vec{S}_1 \cdot \vec{a}_1 \vec{S}_1 \cdot \vec{v}_2 + 2 \hat{n} \cdot \vec{S}_1 \hat{n} \cdot \vec{S}_1 \vec{v}_1 \cdot \vec{v}_2 + \frac{7}{2} \vec{S}_1 \cdot \vec{S}_1 \vec{v}_1 \cdot \vec{v}_2 + \frac{7}{2} \vec{S}_1 \cdot \vec{S}_1 \vec{v}_1 \cdot \vec{v}_2 \Big) + \\
& \frac{1}{r^3} \Big( 8 \hat{n} \cdot \vec{a}_1 \hat{n} \cdot \vec{v}_1 \hat{n} \cdot \vec{v}_2 (\hat{n} \cdot \vec{S}_1)^2 - \frac{4}{3} \hat{n} \cdot \vec{v}_1 \vec{a}_1 \cdot \vec{v}_2 (\hat{n} \cdot \vec{S}_1)^2 - \frac{4}{3} \hat{n} \cdot \vec{v}_2 \vec{v}_1 \cdot \vec{a}_1 (\hat{n} \cdot \vec{S}_1)^2 - \\
& \frac{4}{3} \hat{n} \cdot \vec{a}_1 \vec{v}_1 \cdot \vec{v}_2 (\hat{n} \cdot \vec{S}_1)^2 + 20 \hat{n} \cdot \vec{S}_1 (\hat{n} \cdot \vec{v}_1)^2 \hat{n} \cdot \vec{v}_2 \hat{n} \cdot \vec{S}_1 - \frac{32}{3} \hat{n} \cdot \vec{v}_1 \hat{n} \cdot \vec{v}_2 \vec{S}_1 \cdot \vec{v}_1 \hat{n} \cdot \vec{S}_1 - \\
& \frac{10}{3} (\hat{n} \cdot \vec{v}_1)^2 \vec{S}_1 \cdot \vec{v}_2 \hat{n} \cdot \vec{S}_1 - \frac{14}{3} \hat{n} \cdot \vec{v}_1 \hat{n} \cdot \vec{v}_2 \vec{S}_1 \cdot \vec{a}_1 \hat{n} \cdot \vec{S}_1 - \frac{14}{3} \hat{n} \cdot \vec{a}_1 \hat{n} \cdot \vec{v}_2 \vec{S}_1 \cdot \vec{v}_1 \hat{n} \cdot \vec{S}_1 + \frac{7}{6} \vec{a}_1 \cdot \vec{v}_2 \vec{S}_1 \cdot \vec{v}_1 \hat{n} \cdot \vec{S}_1 - \\
& \frac{8}{3} \hat{n} \cdot \vec{a}_1 \hat{n} \cdot \vec{v}_1 \vec{S}_1 \cdot \vec{v}_2 \hat{n} \cdot \vec{S}_1 + \frac{2}{3} \vec{S}_1 \cdot \vec{v}_2 \vec{v}_1 \cdot \vec{a}_1 \hat{n} \cdot \vec{S}_1 - \frac{10}{3} \hat{n} \cdot \vec{S}_1 \hat{n} \cdot \vec{v}_2 \vec{v}_1 \cdot \vec{v}_1 \hat{n} \cdot \vec{S}_1 + \frac{5}{6} \vec{S}_1 \cdot \vec{v}_2 \vec{v}_1 \cdot \vec{v}_1 \hat{n} \cdot \vec{S}_1 - \\
& \frac{20}{3} \hat{n} \cdot \vec{S}_1 \hat{n} \cdot \vec{v}_1 \vec{v}_1 \cdot \vec{v}_2 \hat{n} \cdot \vec{S}_1 + \frac{8}{3} \vec{S}_1 \cdot \vec{v}_1 \vec{v}_1 \cdot \vec{v}_2 \hat{n} \cdot \vec{S}_1 + \frac{7}{6} \vec{S}_1 \cdot \vec{a}_1 \vec{v}_1 \cdot \vec{v}_2 \hat{n} \cdot \vec{S}_1 + \frac{56}{3} (\hat{n} \cdot \vec{v}_1)^2 \hat{n} \cdot \vec{v}_2 \vec{S}_1 \cdot \vec{S}_1 + \\
& \frac{20}{3} \hat{n} \cdot \vec{a}_1 \hat{n} \cdot \vec{v}_1 \hat{n} \cdot \vec{v}_2 \vec{S}_1 \cdot \vec{S}_1 - \frac{5}{3} \hat{n} \cdot \vec{v}_1 \vec{a}_1 \cdot \vec{v}_2 \vec{S}_1 \cdot \vec{S}_1 - \frac{32}{3} \hat{n} \cdot \vec{S}_1 \hat{n} \cdot \vec{v}_1 \hat{n} \cdot \vec{v}_2 \vec{S}_1 \cdot \vec{v}_1 + \frac{11}{3} \hat{n} \cdot \vec{v}_2 \vec{S}_1 \cdot \vec{v}_1 \vec{S}_1 \cdot \vec{v}_1 + \\
& \frac{8}{3} \hat{n} \cdot \vec{v}_1 \vec{S}_1 \cdot \vec{v}_2 \vec{S}_1 \cdot \vec{v}_1 + \frac{5}{3} \hat{n} \cdot \vec{v}_2 \vec{S}_1 \cdot \vec{a}_1 \vec{S}_1 \cdot \vec{v}_1 - \frac{10}{3} \hat{n} \cdot \vec{S}_1 (\hat{n} \cdot \vec{v}_1)^2 \vec{S}_1 \cdot \vec{v}_2 + \frac{8}{3} \hat{n} \cdot \vec{v}_1 \vec{S}_1 \cdot \vec{v}_1 \vec{S}_1 \cdot \vec{v}_2 + \\
& \frac{7}{6} \hat{n} \cdot \vec{v}_1 \vec{S}_1 \cdot \vec{a}_1 \vec{S}_1 \cdot \vec{v}_2 + \frac{7}{6} \hat{n} \cdot \vec{a}_1 \vec{S}_1 \cdot \vec{v}_1 \vec{S}_1 \cdot \vec{v}_2 - \frac{5}{3} \hat{n} \cdot \vec{v}_2 \vec{S}_1 \cdot \vec{S}_1 \vec{v}_1 \cdot \vec{a}_1 - \frac{14}{3} \hat{n} \cdot \vec{v}_2 \vec{S}_1 \cdot \vec{S}_1 \vec{v}_1 \cdot \vec{v}_1 + \\
& \frac{5}{6} \hat{n} \cdot \vec{S}_1 \vec{S}_1 \cdot \vec{v}_2 \vec{v}_1 \cdot \vec{v}_1 - \frac{28}{3} \hat{n} \cdot \vec{v}_1 \vec{S}_1 \cdot \vec{S}_1 \vec{v}_1 \cdot \vec{v}_2 - \frac{5}{3} \hat{n} \cdot \vec{a}_1 \vec{S}_1 \cdot \vec{S}_1 \vec{v}_1 \cdot \vec{v}_2 + \frac{8}{3} \hat{n} \cdot \vec{S}_1 \vec{S}_1 \cdot \vec{v}_1 \vec{v}_1 \cdot \vec{v}_2 \Big) + \\
& \frac{1}{r^4} \Big( -16 (\hat{n} \cdot \vec{S}_1)^2 \hat{n} \cdot \vec{v}_2 (\hat{n} \cdot \vec{v}_1)^3 - 4 \hat{n} \cdot \vec{v}_2 \vec{S}_1 \cdot \vec{S}_1 (\hat{n} \cdot \vec{v}_1)^3 + 4 \hat{n} \cdot \vec{S}_1 \vec{S}_1 \cdot \vec{v}_2 (\hat{n} \cdot \vec{v}_1)^3 + \\
& 24 \hat{n} \cdot \vec{S}_1 \hat{n} \cdot \vec{v}_2 \vec{S}_1 \cdot \vec{v}_1 (\hat{n} \cdot \vec{v}_1)^2 - 4 \vec{S}_1 \cdot \vec{v}_1 \vec{S}_1 \cdot \vec{v}_2 (\hat{n} \cdot \vec{v}_1)^2 + 6 (\hat{n} \cdot \vec{S}_1)^2 \vec{v}_1 \cdot \vec{v}_2 (\hat{n} \cdot \vec{v}_1)^2 + \\
& 2 \vec{S}_1 \cdot \vec{S}_1 \vec{v}_1 \cdot \vec{v}_2 (\hat{n} \cdot \vec{v}_1)^2 - 6 \hat{n} \cdot \vec{v}_2 (\vec{S}_1 \cdot \vec{v}_1)^2 \hat{n} \cdot \vec{v}_1 + 6 (\hat{n} \cdot \vec{S}_1)^2 \hat{n} \cdot \vec{v}_2 \vec{v}_1 \cdot \vec{v}_1 \hat{n} \cdot \vec{v}_1 + 2 \hat{n} \cdot \vec{v}_2 \vec{S}_1 \cdot \vec{S}_1 \vec{v}_1 \cdot \vec{v}_1 \hat{n} \cdot \vec{v}_1 - \\
& 2 \hat{n} \cdot \vec{S}_1 \vec{S}_1 \cdot \vec{v}_2 \vec{v}_1 \cdot \vec{v}_1 \hat{n} \cdot \vec{v}_1 - 8 \hat{n} \cdot \vec{S}_1 \vec{S}_1 \cdot \vec{v}_1 \vec{v}_1 \cdot \vec{v}_2 \hat{n} \cdot \vec{v}_1 - 4 \hat{n} \cdot \vec{S}_1 \hat{n} \cdot \vec{v}_2 \vec{S}_1 \cdot \vec{v}_1 \vec{v}_1 \cdot \vec{v}_1 + \\
& \vec{S}_1 \cdot \vec{v}_1 \vec{S}_1 \cdot \vec{v}_2 \vec{v}_1 \cdot \vec{v}_1 + \frac{3}{2} (\vec{S}_1 \cdot \vec{v}_1)^2 \vec{v}_1 \cdot \vec{v}_2 - (\hat{n} \cdot \vec{S}_1)^2 \vec{v}_1 \cdot \vec{v}_1 \vec{v}_1 \cdot \vec{v}_2 - \frac{1}{2} \vec{S}_1 \cdot \vec{S}_1 \vec{v}_1 \cdot \vec{v}_1 \vec{v}_1 \cdot \vec{v}_2 \Big) \Big\} m_2 C_{ES^2_1} \Big\}
\end{aligned}$$

{DiagS1CES2[2, 2, 52],

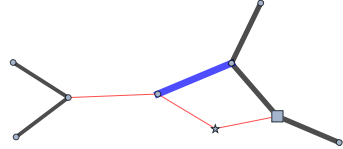

$$\begin{aligned}
& G^2 \left( \frac{1}{r^2} \left( 4 \hat{n} \cdot \vec{S}_1 \hat{n} \cdot \vec{a}_1 \hat{n} \cdot \vec{S}_1 \hat{n} \cdot \vec{v}_1 - \frac{3}{2} \hat{n} \cdot \vec{S}_1 \vec{S}_1 \cdot \vec{a}_1 \hat{n} \cdot \vec{v}_1 + 6 \hat{n} \cdot \vec{a}_1 \vec{S}_1 \cdot \vec{S}_1 \hat{n} \cdot \vec{v}_1 - \frac{3}{2} \hat{n} \cdot \vec{S}_1 \vec{S}_1 \cdot \vec{a}_1 \hat{n} \cdot \vec{v}_1 - \frac{3}{2} \hat{n} \cdot \vec{a}_1 \hat{n} \cdot \vec{S}_1 \right. \right. \\
& \left. \left. \vec{S}_1 \cdot \vec{v}_1 + \vec{S}_1 \cdot \vec{v}_1 \vec{S}_1 \cdot \vec{a}_1 - \frac{3}{2} \hat{n} \cdot \vec{S}_1 \hat{n} \cdot \vec{a}_1 \vec{S}_1 \cdot \vec{v}_1 + \vec{S}_1 \cdot \vec{a}_1 \vec{S}_1 \cdot \vec{v}_1 - \hat{n} \cdot \vec{S}_1 \hat{n} \cdot \vec{S}_1 \vec{v}_1 \cdot \vec{a}_1 - 3 \vec{S}_1 \cdot \vec{S}_1 \vec{v}_1 \cdot \vec{a}_1 \right) + \frac{1}{r^3} \right. \\
& \left( -2 \hat{n} \cdot \vec{S}_1 \hat{n} \cdot \vec{S}_1 (\hat{n} \cdot \vec{v}_1)^3 - \frac{8}{3} \vec{S}_1 \cdot \vec{S}_1 (\hat{n} \cdot \vec{v}_1)^3 - 10 \hat{n} \cdot \vec{a}_1 (\hat{n} \cdot \vec{S}_1)^2 (\hat{n} \cdot \vec{v}_1)^2 + 12 \hat{n} \cdot \vec{S}_1 \hat{n} \cdot \vec{S}_1 \hat{n} \cdot \vec{v}_2 (\hat{n} \cdot \vec{v}_1)^2 + \right. \\
& \left. \hat{n} \cdot \vec{S}_1 \vec{S}_1 \cdot \vec{v}_1 (\hat{n} \cdot \vec{v}_1)^2 - 2 \hat{n} \cdot \vec{S}_1 \vec{S}_1 \cdot \vec{v}_2 (\hat{n} \cdot \vec{v}_1)^2 + 12 \hat{n} \cdot \vec{v}_2 \vec{S}_1 \cdot \vec{S}_1 (\hat{n} \cdot \vec{v}_1)^2 + \frac{13}{3} \hat{n} \cdot \vec{S}_1 \vec{S}_1 \cdot \vec{a}_1 (\hat{n} \cdot \vec{v}_1)^2 - \right. \\
& \left. \frac{28}{3} \hat{n} \cdot \vec{a}_1 \vec{S}_1 \cdot \vec{S}_1 (\hat{n} \cdot \vec{v}_1)^2 + \hat{n} \cdot \vec{S}_1 \vec{S}_1 \cdot \vec{v}_1 (\hat{n} \cdot \vec{v}_1)^2 - 2 \hat{n} \cdot \vec{S}_1 \vec{S}_1 \cdot \vec{v}_2 (\hat{n} \cdot \vec{v}_1)^2 - 6 \hat{n} \cdot \vec{S}_1 \hat{n} \cdot \vec{v}_2 \vec{S}_1 \cdot \vec{v}_1 \hat{n} \cdot \vec{v}_1 + \right. \\
& \left. \frac{29}{3} \hat{n} \cdot \vec{a}_1 \hat{n} \cdot \vec{S}_1 \vec{S}_1 \cdot \vec{v}_1 \hat{n} \cdot \vec{v}_1 - 6 \hat{n} \cdot \vec{S}_1 \hat{n} \cdot \vec{v}_2 \vec{S}_1 \cdot \vec{v}_1 \hat{n} \cdot \vec{v}_1 - \frac{1}{3} \vec{S}_1 \cdot \vec{v}_1 \vec{S}_1 \cdot \vec{v}_1 \hat{n} \cdot \vec{v}_1 + \right. \\
& \left. \frac{3}{2} \vec{S}_1 \cdot \vec{v}_2 \vec{S}_1 \cdot \vec{v}_1 \hat{n} \cdot \vec{v}_1 - \frac{8}{3} \vec{S}_1 \cdot \vec{a}_1 \vec{S}_1 \cdot \vec{v}_1 \hat{n} \cdot \vec{v}_1 + \frac{3}{2} \vec{S}_1 \cdot \vec{v}_1 \vec{S}_1 \cdot \vec{v}_2 \hat{n} \cdot \vec{v}_1 + \frac{23}{6} (\hat{n} \cdot \vec{S}_1)^2 \vec{v}_1 \cdot \vec{a}_1 \hat{n} \cdot \vec{v}_1 + \right. \\
& \left. \frac{25}{6} \vec{S}_1 \cdot \vec{S}_1 \vec{v}_1 \cdot \vec{a}_1 \hat{n} \cdot \vec{v}_1 + 3 \vec{S}_1 \cdot \vec{S}_1 \vec{v}_1 \cdot \vec{v}_1 \hat{n} \cdot \vec{v}_1 - 4 \hat{n} \cdot \vec{S}_1 \hat{n} \cdot \vec{S}_1 \vec{v}_1 \cdot \vec{v}_2 \hat{n} \cdot \vec{v}_1 - 6 \vec{S}_1 \cdot \vec{S}_1 \vec{v}_1 \cdot \vec{v}_2 \hat{n} \cdot \vec{v}_1 - \right. \\
& \left. \frac{4}{3} \hat{n} \cdot \vec{a}_1 (\vec{S}_1 \cdot \vec{v}_1)^2 + 2 \hat{n} \cdot \vec{v}_2 \vec{S}_1 \cdot \vec{v}_1 \vec{S}_1 \cdot \vec{v}_1 - \frac{8}{3} \hat{n} \cdot \vec{S}_1 \vec{S}_1 \cdot \vec{v}_1 \vec{v}_1 \cdot \vec{a}_1 + \frac{13}{6} \hat{n} \cdot \vec{a}_1 (\hat{n} \cdot \vec{S}_1)^2 \vec{v}_1 \cdot \vec{v}_1 - \right.
\end{aligned}$$

$$\begin{aligned}
& 2 \hat{n} \cdot \vec{S}_1 \hat{n} \cdot \vec{S}_1 \hat{n} \cdot \vec{v}_2 \vec{v}_1 \cdot \vec{v}_1 + \frac{1}{2} \hat{n} \cdot \vec{S}_1 \vec{S}_1 \cdot \vec{v}_2 \vec{v}_1 \cdot \vec{v}_1 - 3 \hat{n} \cdot \vec{v}_2 \vec{S}_1 \cdot \vec{S}_1 \vec{v}_1 \cdot \vec{v}_1 - \frac{4}{3} \hat{n} \cdot \vec{S}_1 \vec{S}_1 \cdot \vec{a}_1 \vec{v}_1 \cdot \vec{v}_1 + \\
& \frac{11}{6} \hat{n} \cdot \vec{a}_1 \vec{S}_1 \cdot \vec{S}_1 \vec{v}_1 \cdot \vec{v}_1 + \frac{1}{2} \hat{n} \cdot \vec{S}_1 \vec{S}_1 \cdot \vec{v}_2 \vec{v}_1 \cdot \vec{v}_1 + \frac{3}{2} \hat{n} \cdot \vec{S}_1 \vec{S}_1 \cdot \vec{v}_1 \vec{v}_1 \cdot \vec{v}_2 + \frac{3}{2} \hat{n} \cdot \vec{S}_1 \vec{S}_1 \cdot \vec{v}_1 \vec{v}_1 \cdot \vec{v}_2 \Big) + \frac{1}{r^4} \\
& \left( 5 \left( \hat{n} \cdot \vec{S}_1 \right)^2 \left( \hat{n} \cdot \vec{v}_1 \right)^4 + \frac{17}{4} \vec{S}_1 \cdot \vec{S}_1 \left( \hat{n} \cdot \vec{v}_1 \right)^4 - 40 \left( \hat{n} \cdot \vec{S}_1 \right)^2 \hat{n} \cdot \vec{v}_2 \left( \hat{n} \cdot \vec{v}_1 \right)^3 - 28 \hat{n} \cdot \vec{v}_2 \vec{S}_1 \cdot \vec{S}_1 \left( \hat{n} \cdot \vec{v}_1 \right)^3 - \right. \\
& \frac{23}{4} \hat{n} \cdot \vec{S}_1 \vec{S}_1 \cdot \vec{v}_1 \left( \hat{n} \cdot \vec{v}_1 \right)^3 + 10 \hat{n} \cdot \vec{S}_1 \vec{S}_1 \cdot \vec{v}_2 \left( \hat{n} \cdot \vec{v}_1 \right)^3 + \frac{7}{4} \left( \vec{S}_1 \cdot \vec{v}_1 \right)^2 \left( \hat{n} \cdot \vec{v}_1 \right)^2 + \\
& 42 \hat{n} \cdot \vec{S}_1 \hat{n} \cdot \vec{v}_2 \vec{S}_1 \cdot \vec{v}_1 \left( \hat{n} \cdot \vec{v}_1 \right)^2 - 7 \vec{S}_1 \cdot \vec{v}_1 \vec{S}_1 \cdot \vec{v}_2 \left( \hat{n} \cdot \vec{v}_1 \right)^2 - \frac{9}{8} \left( \hat{n} \cdot \vec{S}_1 \right)^2 \vec{v}_1 \cdot \vec{v}_1 \left( \hat{n} \cdot \vec{v}_1 \right)^2 - \\
& \frac{45}{8} \vec{S}_1 \cdot \vec{S}_1 \vec{v}_1 \cdot \vec{v}_1 \left( \hat{n} \cdot \vec{v}_1 \right)^2 + 15 \left( \hat{n} \cdot \vec{S}_1 \right)^2 \vec{v}_1 \cdot \vec{v}_2 \left( \hat{n} \cdot \vec{v}_1 \right)^2 + 14 \vec{S}_1 \cdot \vec{S}_1 \vec{v}_1 \cdot \vec{v}_2 \left( \hat{n} \cdot \vec{v}_1 \right)^2 - \\
& 8 \hat{n} \cdot \vec{v}_2 \left( \vec{S}_1 \cdot \vec{v}_1 \right)^2 \hat{n} \cdot \vec{v}_1 + 18 \left( \hat{n} \cdot \vec{S}_1 \right)^2 \hat{n} \cdot \vec{v}_2 \vec{v}_1 \cdot \vec{v}_1 \hat{n} \cdot \vec{v}_1 + 12 \hat{n} \cdot \vec{v}_2 \vec{S}_1 \cdot \vec{S}_1 \vec{v}_1 \cdot \vec{v}_1 \hat{n} \cdot \vec{v}_1 + \\
& \frac{9}{4} \hat{n} \cdot \vec{S}_1 \vec{S}_1 \cdot \vec{v}_1 \vec{v}_1 \cdot \vec{v}_1 \hat{n} \cdot \vec{v}_1 - 6 \hat{n} \cdot \vec{S}_1 \vec{S}_1 \cdot \vec{v}_2 \vec{v}_1 \cdot \vec{v}_1 \hat{n} \cdot \vec{v}_1 - 14 \hat{n} \cdot \vec{S}_1 \vec{S}_1 \cdot \vec{v}_1 \vec{v}_1 \cdot \vec{v}_2 \hat{n} \cdot \vec{v}_1 - \\
& \frac{1}{8} \left( \hat{n} \cdot \vec{S}_1 \right)^2 \left( \vec{v}_1 \cdot \vec{v}_1 \right)^2 + \frac{7}{8} \vec{S}_1 \cdot \vec{S}_1 \left( \vec{v}_1 \cdot \vec{v}_1 \right)^2 - \frac{1}{2} \left( \vec{S}_1 \cdot \vec{v}_1 \right)^2 \vec{v}_1 \cdot \vec{v}_1 - 8 \hat{n} \cdot \vec{S}_1 \hat{n} \cdot \vec{v}_2 \vec{S}_1 \cdot \vec{v}_1 \vec{v}_1 \cdot \vec{v}_1 + \\
& 2 \vec{S}_1 \cdot \vec{v}_1 \vec{S}_1 \cdot \vec{v}_2 \vec{v}_1 \cdot \vec{v}_1 + 2 \left( \vec{S}_1 \cdot \vec{v}_1 \right)^2 \vec{v}_1 \cdot \vec{v}_2 - 3 \left( \hat{n} \cdot \vec{S}_1 \right)^2 \vec{v}_1 \cdot \vec{v}_1 \vec{v}_1 \cdot \vec{v}_2 - 3 \vec{S}_1 \cdot \vec{S}_1 \vec{v}_1 \cdot \vec{v}_1 \vec{v}_1 \cdot \vec{v}_2 \Big) \Big) m_2 C_{ES^2 1} \Big\}
\end{aligned}$$

$$\left\{ \text{DiagS1CES2}[2, 2, 53], \right.$$
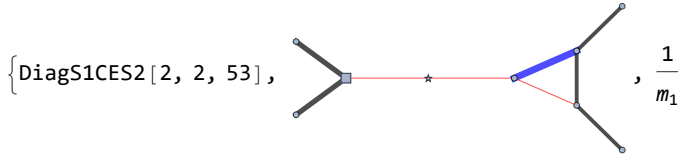

$$, \frac{1}{m_1}$$

$$\begin{aligned}
& G^2 \left( \frac{1}{r^2} \left( \frac{32}{3} \hat{n} \cdot \vec{S}_1 \hat{n} \cdot \vec{a}_2 \hat{n} \cdot \vec{S}_1 \hat{n} \cdot \vec{v}_2 - \frac{8}{3} \hat{n} \cdot \vec{S}_1 \vec{S}_1 \cdot \vec{a}_2 \hat{n} \cdot \vec{v}_2 + \frac{16}{3} \hat{n} \cdot \vec{a}_2 \vec{S}_1 \cdot \vec{S}_1 \hat{n} \cdot \vec{v}_2 - \frac{8}{3} \hat{n} \cdot \vec{S}_1 \vec{S}_1 \cdot \vec{a}_2 \hat{n} \cdot \vec{v}_2 - \frac{8}{3} \hat{n} \cdot \vec{a}_2 \hat{n} \cdot \vec{S}_1 \right. \right. \\
& \left. \left. \vec{S}_1 \cdot \vec{v}_2 + \frac{4}{3} \vec{S}_1 \cdot \vec{v}_2 \vec{S}_1 \cdot \vec{a}_2 - \frac{8}{3} \hat{n} \cdot \vec{S}_1 \hat{n} \cdot \vec{a}_2 \vec{S}_1 \cdot \vec{v}_2 + \frac{4}{3} \vec{S}_1 \cdot \vec{a}_2 \vec{S}_1 \cdot \vec{v}_2 - \frac{8}{3} \hat{n} \cdot \vec{S}_1 \hat{n} \cdot \vec{S}_1 \vec{v}_2 \cdot \vec{a}_2 - \frac{8}{3} \vec{S}_1 \cdot \vec{S}_1 \vec{v}_2 \cdot \vec{a}_2 \right) + \right. \\
& \frac{1}{r^3} \left( 32 \hat{n} \cdot \vec{S}_1 \hat{n} \cdot \vec{S}_1 \left( \hat{n} \cdot \vec{v}_2 \right)^3 + \frac{32}{3} \vec{S}_1 \cdot \vec{S}_1 \left( \hat{n} \cdot \vec{v}_2 \right)^3 - 16 \hat{n} \cdot \vec{S}_1 \vec{S}_1 \cdot \vec{v}_2 \left( \hat{n} \cdot \vec{v}_2 \right)^2 - 16 \hat{n} \cdot \vec{S}_1 \vec{S}_1 \cdot \vec{v}_2 \left( \hat{n} \cdot \vec{v}_2 \right)^2 - \right. \\
& 32 \hat{n} \cdot \vec{a}_2 \left( \hat{n} \cdot \vec{S}_1 \right)^2 \hat{n} \cdot \vec{v}_1 \hat{n} \cdot \vec{v}_2 + \frac{32}{3} \hat{n} \cdot \vec{S}_1 \hat{n} \cdot \vec{v}_1 \vec{S}_1 \cdot \vec{a}_2 \hat{n} \cdot \vec{v}_2 - \frac{32}{3} \hat{n} \cdot \vec{a}_2 \hat{n} \cdot \vec{v}_1 \vec{S}_1 \cdot \vec{S}_1 \hat{n} \cdot \vec{v}_2 + \\
& \frac{32}{3} \hat{n} \cdot \vec{a}_2 \hat{n} \cdot \vec{S}_1 \vec{S}_1 \cdot \vec{v}_1 \hat{n} \cdot \vec{v}_2 - \frac{8}{3} \vec{S}_1 \cdot \vec{a}_2 \vec{S}_1 \cdot \vec{v}_1 \hat{n} \cdot \vec{v}_2 + 8 \vec{S}_1 \cdot \vec{v}_2 \vec{S}_1 \cdot \vec{v}_2 \hat{n} \cdot \vec{v}_2 + \\
& \frac{16}{3} \left( \hat{n} \cdot \vec{S}_1 \right)^2 \vec{v}_1 \cdot \vec{a}_2 \hat{n} \cdot \vec{v}_2 + \frac{8}{3} \vec{S}_1 \cdot \vec{S}_1 \vec{v}_1 \cdot \vec{a}_2 \hat{n} \cdot \vec{v}_2 - 16 \hat{n} \cdot \vec{S}_1 \hat{n} \cdot \vec{S}_1 \vec{v}_2 \cdot \vec{v}_2 \hat{n} \cdot \vec{v}_2 - 8 \vec{S}_1 \cdot \vec{S}_1 \vec{v}_2 \cdot \vec{v}_2 \hat{n} \cdot \vec{v}_2 + \\
& \frac{32}{3} \hat{n} \cdot \vec{a}_2 \hat{n} \cdot \vec{S}_1 \hat{n} \cdot \vec{v}_1 \vec{S}_1 \cdot \vec{v}_2 - \frac{8}{3} \hat{n} \cdot \vec{v}_1 \vec{S}_1 \cdot \vec{a}_2 \vec{S}_1 \cdot \vec{v}_2 - \frac{8}{3} \hat{n} \cdot \vec{a}_2 \vec{S}_1 \cdot \vec{v}_1 \vec{S}_1 \cdot \vec{v}_2 - \frac{8}{3} \hat{n} \cdot \vec{S}_1 \vec{S}_1 \cdot \vec{v}_2 \vec{v}_1 \cdot \vec{a}_2 + \\
& \frac{16}{3} \hat{n} \cdot \vec{a}_2 \left( \hat{n} \cdot \vec{S}_1 \right)^2 \vec{v}_1 \cdot \vec{v}_2 - \frac{8}{3} \hat{n} \cdot \vec{S}_1 \vec{S}_1 \cdot \vec{a}_2 \vec{v}_1 \cdot \vec{v}_2 + \frac{8}{3} \hat{n} \cdot \vec{a}_2 \vec{S}_1 \cdot \vec{S}_1 \vec{v}_1 \cdot \vec{v}_2 + \frac{16}{3} \left( \hat{n} \cdot \vec{S}_1 \right)^2 \hat{n} \cdot \vec{v}_1 \vec{v}_2 \cdot \vec{a}_2 + \\
& \left. \frac{8}{3} \hat{n} \cdot \vec{v}_1 \vec{S}_1 \cdot \vec{S}_1 \vec{v}_2 \cdot \vec{a}_2 - \frac{8}{3} \hat{n} \cdot \vec{S}_1 \vec{S}_1 \cdot \vec{v}_1 \vec{v}_2 \cdot \vec{a}_2 + 4 \hat{n} \cdot \vec{S}_1 \vec{S}_1 \cdot \vec{v}_2 \vec{v}_2 \cdot \vec{v}_2 + 4 \hat{n} \cdot \vec{S}_1 \vec{S}_1 \cdot \vec{v}_2 \vec{v}_2 \cdot \vec{v}_2 \right) + \\
& \frac{1}{r^4} \left( -128 \left( \hat{n} \cdot \vec{S}_1 \right)^2 \hat{n} \cdot \vec{v}_1 \left( \hat{n} \cdot \vec{v}_2 \right)^3 - 32 \hat{n} \cdot \vec{v}_1 \vec{S}_1 \cdot \vec{S}_1 \left( \hat{n} \cdot \vec{v}_2 \right)^3 + 32 \hat{n} \cdot \vec{S}_1 \vec{S}_1 \cdot \vec{v}_1 \left( \hat{n} \cdot \vec{v}_2 \right)^3 + \right. \\
& 96 \hat{n} \cdot \vec{S}_1 \hat{n} \cdot \vec{v}_1 \vec{S}_1 \cdot \vec{v}_2 \left( \hat{n} \cdot \vec{v}_2 \right)^2 - 16 \vec{S}_1 \cdot \vec{v}_1 \vec{S}_1 \cdot \vec{v}_2 \left( \hat{n} \cdot \vec{v}_2 \right)^2 + 48 \left( \hat{n} \cdot \vec{S}_1 \right)^2 \vec{v}_1 \cdot \vec{v}_2 \left( \hat{n} \cdot \vec{v}_2 \right)^2 + \\
& 16 \vec{S}_1 \cdot \vec{S}_1 \vec{v}_1 \cdot \vec{v}_2 \left( \hat{n} \cdot \vec{v}_2 \right)^2 - 16 \hat{n} \cdot \vec{v}_1 \left( \vec{S}_1 \cdot \vec{v}_2 \right)^2 \hat{n} \cdot \vec{v}_2 - 32 \hat{n} \cdot \vec{S}_1 \vec{S}_1 \cdot \vec{v}_2 \vec{v}_1 \cdot \vec{v}_2 \hat{n} \cdot \vec{v}_2 + \\
& 48 \left( \hat{n} \cdot \vec{S}_1 \right)^2 \hat{n} \cdot \vec{v}_1 \vec{v}_2 \cdot \vec{v}_2 \hat{n} \cdot \vec{v}_2 + 16 \hat{n} \cdot \vec{v}_1 \vec{S}_1 \cdot \vec{S}_1 \vec{v}_2 \cdot \vec{v}_2 \hat{n} \cdot \vec{v}_2 - 16 \hat{n} \cdot \vec{S}_1 \vec{S}_1 \cdot \vec{v}_1 \vec{v}_2 \cdot \vec{v}_2 \hat{n} \cdot \vec{v}_2 + 4 \left( \vec{S}_1 \cdot \vec{v}_2 \right)^2 \vec{v}_1 \cdot \vec{v}_2 - \\
& \left. 16 \hat{n} \cdot \vec{S}_1 \hat{n} \cdot \vec{v}_1 \vec{S}_1 \cdot \vec{v}_2 \vec{v}_2 \cdot \vec{v}_2 + 4 \vec{S}_1 \cdot \vec{v}_1 \vec{S}_1 \cdot \vec{v}_2 \vec{v}_2 \cdot \vec{v}_2 - 8 \left( \hat{n} \cdot \vec{S}_1 \right)^2 \vec{v}_1 \cdot \vec{v}_2 \vec{v}_2 \cdot \vec{v}_2 - 4 \vec{S}_1 \cdot \vec{S}_1 \vec{v}_1 \cdot \vec{v}_2 \vec{v}_2 \cdot \vec{v}_2 \right) \Big) m_2^2 C_{ES^2 1} \Big\}
\end{aligned}$$



{DiagS1CES2[2, 2, 54],

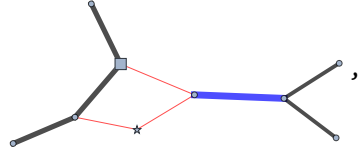

$$\begin{aligned}
 G^2 \left( \frac{1}{\kappa^3} \left( \frac{5}{4} \hat{n} \cdot \vec{a}_2 \hat{n} \cdot \vec{v}_1 \hat{n} \cdot \vec{v}_2 (\hat{n} \cdot \vec{S}_1)^2 - \frac{25}{12} \hat{n} \cdot \vec{v}_2 \vec{v}_1 \cdot \vec{a}_2 (\hat{n} \cdot \vec{S}_1)^2 - \frac{25}{12} \hat{n} \cdot \vec{a}_2 \vec{v}_1 \cdot \vec{v}_2 (\hat{n} \cdot \vec{S}_1)^2 + \right. \right. \\
 \frac{5}{12} \hat{n} \cdot \vec{v}_1 \vec{v}_2 \cdot \vec{a}_2 (\hat{n} \cdot \vec{S}_1)^2 + \frac{5}{4} \hat{n} \cdot \vec{S}_1 \hat{n} \cdot \vec{v}_1 (\hat{n} \cdot \vec{v}_2)^2 \hat{n} \cdot \vec{S}_1 + \frac{5}{12} (\hat{n} \cdot \vec{v}_2)^2 \vec{S}_1 \cdot \vec{v}_1 \hat{n} \cdot \vec{S}_1 - \frac{1}{6} \hat{n} \cdot \vec{v}_1 \hat{n} \cdot \vec{v}_2 \\
 \vec{S}_1 \cdot \vec{v}_2 \hat{n} \cdot \vec{S}_1 - \frac{1}{6} \hat{n} \cdot \vec{v}_1 \hat{n} \cdot \vec{v}_2 \vec{S}_1 \cdot \vec{a}_2 \hat{n} \cdot \vec{S}_1 + \frac{5}{6} \hat{n} \cdot \vec{a}_2 \hat{n} \cdot \vec{v}_2 \vec{S}_1 \cdot \vec{v}_1 \hat{n} \cdot \vec{S}_1 - \frac{1}{6} \hat{n} \cdot \vec{a}_2 \hat{n} \cdot \vec{v}_1 \vec{S}_1 \cdot \vec{v}_2 \hat{n} \cdot \vec{S}_1 + \\
 \frac{2}{3} \vec{S}_1 \cdot \vec{v}_2 \vec{v}_1 \cdot \vec{a}_2 \hat{n} \cdot \vec{S}_1 - \frac{25}{6} \hat{n} \cdot \vec{S}_1 \hat{n} \cdot \vec{v}_2 \vec{v}_1 \cdot \vec{v}_2 \hat{n} \cdot \vec{S}_1 + \frac{2}{3} \vec{S}_1 \cdot \vec{v}_2 \vec{v}_1 \cdot \vec{v}_2 \hat{n} \cdot \vec{S}_1 + \frac{2}{3} \vec{S}_1 \cdot \vec{a}_2 \vec{v}_1 \cdot \vec{v}_2 \hat{n} \cdot \vec{S}_1 - \\
 \frac{5}{6} \vec{S}_1 \cdot \vec{v}_1 \vec{v}_2 \cdot \vec{a}_2 \hat{n} \cdot \vec{S}_1 + \frac{5}{12} \hat{n} \cdot \vec{S}_1 \hat{n} \cdot \vec{v}_1 \vec{v}_2 \cdot \vec{v}_2 \hat{n} \cdot \vec{S}_1 - \frac{5}{12} \vec{S}_1 \cdot \vec{v}_1 \vec{v}_2 \cdot \vec{v}_2 \hat{n} \cdot \vec{S}_1 - \frac{7}{12} \hat{n} \cdot \vec{v}_1 (\hat{n} \cdot \vec{v}_2)^2 \vec{S}_1 \cdot \vec{S}_1 - \\
 \frac{7}{12} \hat{n} \cdot \vec{a}_2 \hat{n} \cdot \vec{v}_1 \hat{n} \cdot \vec{v}_2 \vec{S}_1 \cdot \vec{S}_1 + \frac{5}{12} \hat{n} \cdot \vec{S}_1 (\hat{n} \cdot \vec{v}_2)^2 \vec{S}_1 \cdot \vec{v}_1 - \frac{1}{3} \hat{n} \cdot \vec{v}_2 \vec{S}_1 \cdot \vec{v}_2 \vec{S}_1 \cdot \vec{v}_1 - \frac{1}{3} \hat{n} \cdot \vec{v}_2 \vec{S}_1 \cdot \vec{a}_2 \vec{S}_1 \cdot \vec{v}_1 - \\
 \frac{1}{6} \hat{n} \cdot \vec{S}_1 \hat{n} \cdot \vec{v}_1 \hat{n} \cdot \vec{v}_2 \vec{S}_1 \cdot \vec{v}_2 - \frac{1}{3} \hat{n} \cdot \vec{v}_2 \vec{S}_1 \cdot \vec{v}_1 \vec{S}_1 \cdot \vec{v}_2 + \frac{1}{6} \hat{n} \cdot \vec{v}_1 \vec{S}_1 \cdot \vec{v}_2 \vec{S}_1 \cdot \vec{v}_2 + \frac{1}{6} \hat{n} \cdot \vec{v}_1 \vec{S}_1 \cdot \vec{a}_2 \vec{S}_1 \cdot \vec{v}_2 - \\
 \frac{1}{3} \hat{n} \cdot \vec{a}_2 \vec{S}_1 \cdot \vec{v}_1 \vec{S}_1 \cdot \vec{v}_2 + \frac{7}{12} \hat{n} \cdot \vec{v}_2 \vec{S}_1 \cdot \vec{S}_1 \vec{v}_1 \cdot \vec{a}_2 + \frac{7}{6} \hat{n} \cdot \vec{v}_2 \vec{S}_1 \cdot \vec{S}_1 \vec{v}_1 \cdot \vec{v}_2 + \frac{7}{12} \hat{n} \cdot \vec{a}_2 \vec{S}_1 \cdot \vec{S}_1 \vec{v}_1 \cdot \vec{v}_2 + \\
 \left. \frac{2}{3} \hat{n} \cdot \vec{S}_1 \vec{S}_1 \cdot \vec{v}_2 \vec{v}_1 \cdot \vec{v}_2 + \frac{1}{12} \hat{n} \cdot \vec{v}_1 \vec{S}_1 \cdot \vec{S}_1 \vec{v}_2 \cdot \vec{a}_2 + \frac{1}{12} \hat{n} \cdot \vec{v}_1 \vec{S}_1 \cdot \vec{S}_1 \vec{v}_2 \cdot \vec{v}_2 - \frac{5}{12} \hat{n} \cdot \vec{S}_1 \vec{S}_1 \cdot \vec{v}_1 \vec{v}_2 \cdot \vec{v}_2 \right) + \\
 \frac{1}{\kappa^4} \left( 5 (\hat{n} \cdot \vec{S}_1)^2 \hat{n} \cdot \vec{v}_1 (\hat{n} \cdot \vec{v}_2)^3 - \frac{7}{4} \hat{n} \cdot \vec{v}_1 \vec{S}_1 \cdot \vec{S}_1 (\hat{n} \cdot \vec{v}_2)^3 + \frac{5}{2} \hat{n} \cdot \vec{S}_1 \vec{S}_1 \cdot \vec{v}_1 (\hat{n} \cdot \vec{v}_2)^3 - \right. \\
 \frac{7}{2} (\hat{n} \cdot \vec{S}_1)^2 (\hat{n} \cdot \vec{v}_1)^2 (\hat{n} \cdot \vec{v}_2)^2 - \frac{1}{12} (\vec{S}_1 \cdot \vec{v}_1)^2 (\hat{n} \cdot \vec{v}_2)^2 + (\hat{n} \cdot \vec{v}_1)^2 \vec{S}_1 \cdot \vec{S}_1 (\hat{n} \cdot \vec{v}_2)^2 + \\
 \frac{1}{4} \hat{n} \cdot \vec{S}_1 \hat{n} \cdot \vec{v}_1 \vec{S}_1 \cdot \vec{v}_1 (\hat{n} \cdot \vec{v}_2)^2 - \frac{9}{4} \hat{n} \cdot \vec{S}_1 \hat{n} \cdot \vec{v}_1 \vec{S}_1 \cdot \vec{v}_2 (\hat{n} \cdot \vec{v}_2)^2 - \frac{7}{4} \vec{S}_1 \cdot \vec{v}_1 \vec{S}_1 \cdot \vec{v}_2 (\hat{n} \cdot \vec{v}_2)^2 - \\
 \frac{7}{8} (\hat{n} \cdot \vec{S}_1)^2 \vec{v}_1 \cdot \vec{v}_1 (\hat{n} \cdot \vec{v}_2)^2 - \frac{1}{24} \vec{S}_1 \cdot \vec{S}_1 \vec{v}_1 \cdot \vec{v}_1 (\hat{n} \cdot \vec{v}_2)^2 - \frac{105}{8} (\hat{n} \cdot \vec{S}_1)^2 \vec{v}_1 \cdot \vec{v}_2 (\hat{n} \cdot \vec{v}_2)^2 + \\
 \frac{21}{8} \vec{S}_1 \cdot \vec{S}_1 \vec{v}_1 \cdot \vec{v}_2 (\hat{n} \cdot \vec{v}_2)^2 + \frac{1}{2} \hat{n} \cdot \vec{v}_1 (\vec{S}_1 \cdot \vec{v}_2)^2 \hat{n} \cdot \vec{v}_2 + \frac{1}{4} \hat{n} \cdot \vec{S}_1 (\hat{n} \cdot \vec{v}_1)^2 \vec{S}_1 \cdot \vec{v}_2 \hat{n} \cdot \vec{v}_2 + \\
 \frac{2}{3} \hat{n} \cdot \vec{v}_1 \vec{S}_1 \cdot \vec{v}_1 \vec{S}_1 \cdot \vec{v}_2 \hat{n} \cdot \vec{v}_2 + \frac{13}{12} \hat{n} \cdot \vec{S}_1 \vec{S}_1 \cdot \vec{v}_2 \vec{v}_1 \cdot \vec{v}_1 \hat{n} \cdot \vec{v}_2 + \frac{23}{2} (\hat{n} \cdot \vec{S}_1)^2 \hat{n} \cdot \vec{v}_1 \vec{v}_1 \cdot \vec{v}_2 \hat{n} \cdot \vec{v}_2 - \\
 \frac{13}{6} \hat{n} \cdot \vec{v}_1 \vec{S}_1 \cdot \vec{S}_1 \vec{v}_1 \cdot \vec{v}_2 \hat{n} \cdot \vec{v}_2 - \frac{17}{6} \hat{n} \cdot \vec{S}_1 \vec{S}_1 \cdot \vec{v}_1 \vec{v}_1 \cdot \vec{v}_2 \hat{n} \cdot \vec{v}_2 + 7 \hat{n} \cdot \vec{S}_1 \vec{S}_1 \cdot \vec{v}_2 \vec{v}_1 \cdot \vec{v}_2 \hat{n} \cdot \vec{v}_2 + \\
 \frac{3}{4} \hat{n} \cdot \vec{v}_1 \vec{S}_1 \cdot \vec{S}_1 \vec{v}_2 \cdot \vec{v}_2 \hat{n} \cdot \vec{v}_2 - \frac{5}{2} \hat{n} \cdot \vec{S}_1 \vec{S}_1 \cdot \vec{v}_1 \vec{v}_2 \cdot \vec{v}_2 \hat{n} \cdot \vec{v}_2 - \frac{1}{12} (\hat{n} \cdot \vec{v}_1)^2 (\vec{S}_1 \cdot \vec{v}_2)^2 - \frac{4}{3} (\hat{n} \cdot \vec{S}_1)^2 (\vec{v}_1 \cdot \vec{v}_2)^2 + \\
 \frac{1}{3} \vec{S}_1 \cdot \vec{S}_1 (\vec{v}_1 \cdot \vec{v}_2)^2 - \frac{1}{6} (\vec{S}_1 \cdot \vec{v}_2)^2 \vec{v}_1 \cdot \vec{v}_1 - \frac{3}{4} (\vec{S}_1 \cdot \vec{v}_2)^2 \vec{v}_1 \cdot \vec{v}_2 - \frac{17}{6} \hat{n} \cdot \vec{S}_1 \hat{n} \cdot \vec{v}_1 \vec{S}_1 \cdot \vec{v}_2 \vec{v}_1 \cdot \vec{v}_2 + \\
 \frac{1}{3} \vec{S}_1 \cdot \vec{v}_1 \vec{S}_1 \cdot \vec{v}_2 \vec{v}_1 \cdot \vec{v}_2 - \frac{7}{8} (\hat{n} \cdot \vec{S}_1)^2 (\hat{n} \cdot \vec{v}_1)^2 \vec{v}_2 \cdot \vec{v}_2 - \frac{1}{6} (\vec{S}_1 \cdot \vec{v}_1)^2 \vec{v}_2 \cdot \vec{v}_2 - \frac{1}{24} (\hat{n} \cdot \vec{v}_1)^2 \vec{S}_1 \cdot \vec{S}_1 \vec{v}_2 \cdot \vec{v}_2 + \\
 \frac{13}{12} \hat{n} \cdot \vec{S}_1 \hat{n} \cdot \vec{v}_1 \vec{S}_1 \cdot \vec{v}_1 \vec{v}_2 \cdot \vec{v}_2 - \frac{1}{4} \hat{n} \cdot \vec{S}_1 \hat{n} \cdot \vec{v}_1 \vec{S}_1 \cdot \vec{v}_2 \vec{v}_2 \cdot \vec{v}_2 + \frac{3}{4} \vec{S}_1 \cdot \vec{v}_1 \vec{S}_1 \cdot \vec{v}_2 \vec{v}_2 \cdot \vec{v}_2 + \frac{7}{12} (\hat{n} \cdot \vec{S}_1)^2 \vec{v}_1 \cdot \vec{v}_1 \vec{v}_2 \cdot \vec{v}_2 - \\
 \left. \frac{1}{12} \vec{S}_1 \cdot \vec{S}_1 \vec{v}_1 \cdot \vec{v}_1 \vec{v}_2 \cdot \vec{v}_2 + \frac{15}{8} (\hat{n} \cdot \vec{S}_1)^2 \vec{v}_1 \cdot \vec{v}_2 \vec{v}_2 \cdot \vec{v}_2 - \frac{5}{8} \vec{S}_1 \cdot \vec{S}_1 \vec{v}_1 \cdot \vec{v}_2 \vec{v}_2 \cdot \vec{v}_2 \right) \Bigg) m_2 C_{ES^2 1} \}
 \end{aligned}$$

{DiagS1CES2[2, 2, 55],

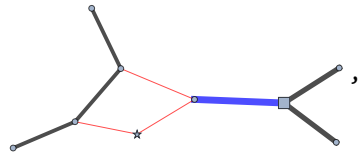

$$\begin{aligned} & \frac{1}{m_1} G^2 \left( \frac{1}{r} \left( -\frac{1}{2} \hat{n} \cdot \vec{S}_1 \hat{n} \cdot \vec{S}_1 \hat{n} \cdot \vec{v}_2 - \frac{1}{6} \hat{n} \cdot \vec{S}_1^3 \hat{n} \cdot \vec{S}_1 \hat{n} \cdot \vec{v}_2 - \frac{1}{2} \vec{S}_1 \cdot \vec{S}_1 \hat{n} \cdot \vec{v}_2 - \right. \right. \\ & \quad \left. \frac{1}{6} \vec{S}_1 \cdot \vec{S}_1 \hat{n} \cdot \vec{v}_2 + \hat{n} \cdot \vec{S}_1^3 \vec{S}_1 \cdot \vec{v}_2 + \hat{n} \cdot \vec{S}_1 \vec{S}_1^2 \cdot \vec{v}_2 + \frac{1}{3} \hat{n} \cdot \vec{S}_1 \vec{S}_1^3 \cdot \vec{v}_2 + \frac{1}{3} \hat{n} \cdot \vec{S}_1^3 \vec{S}_1 \cdot \vec{v}_2 \right) + \frac{1}{r^2} \\ & \quad \left( -\frac{1}{3} (\hat{n} \cdot \vec{v}_2)^2 \left( \hat{n} \cdot \vec{S}_1 \right)^2 + 2 \hat{n} \cdot \vec{v}_1 \hat{n} \cdot \vec{v}_2 \left( \hat{n} \cdot \vec{S}_1 \right)^2 - \frac{3}{2} \vec{v}_1 \cdot \vec{v}_2 \left( \hat{n} \cdot \vec{S}_1 \right)^2 - \frac{1}{6} \vec{v}_2 \cdot \vec{v}_2 \left( \hat{n} \cdot \vec{S}_1 \right)^2 + \right. \\ & \quad 2 \hat{n} \cdot \vec{a}_1 \hat{n} \cdot \vec{S}_1 \hat{n} \cdot \vec{v}_2 \hat{n} \cdot \vec{S}_1 - 3 \hat{n} \cdot \vec{v}_1 \vec{S}_1 \cdot \vec{v}_2 \hat{n} \cdot \vec{S}_1 + \frac{4}{3} \hat{n} \cdot \vec{v}_2 \vec{S}_1 \cdot \vec{v}_2 \hat{n} \cdot \vec{S}_1 - \frac{5}{2} \hat{n} \cdot \vec{S}_1 \vec{a}_1 \cdot \vec{v}_2 \hat{n} \cdot \vec{S}_1 + \\ & \quad \frac{1}{2} \hat{n} \cdot \vec{v}_2 \vec{S}_1 \cdot \vec{a}_1 \hat{n} \cdot \vec{S}_1 - \hat{n} \cdot \vec{a}_1 \vec{S}_1 \cdot \vec{v}_2 \hat{n} \cdot \vec{S}_1 - \frac{1}{3} \hat{n} \cdot \vec{S}_1^2 \hat{n} \cdot \vec{S}_1 (\hat{n} \cdot \vec{v}_2)^2 - \frac{1}{3} \left( \vec{S}_1 \cdot \vec{v}_2 \right)^2 + \frac{1}{3} \hat{n} \cdot \vec{a}_1 (\hat{n} \cdot \vec{S}_1)^2 \hat{n} \cdot \vec{v}_2 + \\ & \quad 2 \hat{n} \cdot \vec{S}_1^2 \hat{n} \cdot \vec{S}_1 \hat{n} \cdot \vec{v}_1 \hat{n} \cdot \vec{v}_2 - \frac{7}{12} (\hat{n} \cdot \vec{S}_1)^2 \vec{a}_1 \cdot \vec{v}_2 - \frac{2}{3} (\hat{n} \cdot \vec{v}_2)^2 \vec{S}_1 \cdot \vec{S}_1 + \hat{n} \cdot \vec{v}_1 \hat{n} \cdot \vec{v}_2 \vec{S}_1 \cdot \vec{S}_1 + \\ & \quad \frac{1}{2} \hat{n} \cdot \vec{S}_1 \hat{n} \cdot \vec{v}_2 \vec{S}_1 \cdot \vec{a}_1 - \hat{n} \cdot \vec{a}_1 \hat{n} \cdot \vec{S}_1 \vec{S}_1 \cdot \vec{v}_2 + \vec{S}_1 \cdot \vec{v}_1 \vec{S}_1 \cdot \vec{v}_2 - \frac{3}{2} \hat{n} \cdot \vec{S}_1 \hat{n} \cdot \vec{v}_1 \vec{S}_1 \cdot \vec{v}_2 + \frac{2}{3} \hat{n} \cdot \vec{S}_1 \hat{n} \cdot \vec{v}_2 \vec{S}_1 \cdot \vec{v}_2 + \\ & \quad \frac{1}{3} \hat{n} \cdot \vec{S}_1 \hat{n} \cdot \vec{v}_2 \vec{S}_1 \cdot \vec{a}_1 + \hat{n} \cdot \vec{a}_1 \hat{n} \cdot \vec{v}_2 \vec{S}_1 \cdot \vec{S}_1 - \frac{1}{2} \vec{a}_1 \cdot \vec{v}_2 \vec{S}_1 \cdot \vec{S}_1 - \frac{2}{3} (\hat{n} \cdot \vec{v}_2)^2 \vec{S}_1 \cdot \vec{S}_1 + \hat{n} \cdot \vec{v}_1 \hat{n} \cdot \vec{v}_2 \vec{S}_1 \cdot \vec{S}_1 + \\ & \quad \frac{1}{6} \hat{n} \cdot \vec{a}_1 \hat{n} \cdot \vec{v}_2 \vec{S}_1 \cdot \vec{S}_1 - \frac{1}{12} \vec{a}_1 \cdot \vec{v}_2 \vec{S}_1 \cdot \vec{S}_1 + \frac{1}{2} \vec{S}_1^2 \cdot \vec{v}_2 \vec{S}_1 \cdot \vec{v}_1 - \frac{1}{6} \hat{n} \cdot \vec{a}_1 \hat{n} \cdot \vec{S}_1 \vec{S}_1 \cdot \vec{v}_2 - \frac{3}{2} \hat{n} \cdot \vec{S}_1^2 \hat{n} \cdot \vec{v}_1 \vec{S}_1 \cdot \vec{v}_2 + \\ & \quad \frac{2}{3} \hat{n} \cdot \vec{S}_1^2 \hat{n} \cdot \vec{v}_2 \vec{S}_1 \cdot \vec{v}_2 + \frac{1}{2} \vec{S}_1 \cdot \vec{v}_1 \vec{S}_1 \cdot \vec{v}_2 - \frac{1}{3} \vec{S}_1^2 \cdot \vec{v}_2 \vec{S}_1 \cdot \vec{v}_2 - \frac{1}{6} \vec{S}_1 \cdot \vec{a}_1 \vec{S}_1 \cdot \vec{v}_2 - \frac{3}{2} \hat{n} \cdot \vec{S}_1^2 \hat{n} \cdot \vec{S}_1 \vec{v}_1 \cdot \vec{v}_2 - \\ & \quad \left. \frac{1}{2} \vec{S}_1 \cdot \vec{S}_1 \vec{v}_1 \cdot \vec{v}_2 - \frac{1}{2} \vec{S}_1 \cdot \vec{S}_1 \vec{v}_1 \cdot \vec{v}_2 - \frac{1}{6} \hat{n} \cdot \vec{S}_1 \hat{n} \cdot \vec{S}_1 \vec{v}_2 \cdot \vec{v}_2 - \frac{1}{6} \vec{S}_1 \cdot \vec{S}_1 \vec{v}_2 \cdot \vec{v}_2 - \frac{1}{6} \vec{S}_1 \cdot \vec{S}_1 \vec{v}_2 \cdot \vec{v}_2 \right) + \\ & \quad \frac{1}{r^3} \left( \hat{n} \cdot \vec{a}_1 (\hat{n} \cdot \vec{v}_2)^2 (\hat{n} \cdot \vec{S}_1)^2 - 6 \hat{n} \cdot \vec{a}_1 \hat{n} \cdot \vec{v}_1 \hat{n} \cdot \vec{v}_2 (\hat{n} \cdot \vec{S}_1)^2 + 5 \hat{n} \cdot \vec{v}_1 \vec{a}_1 \cdot \vec{v}_2 (\hat{n} \cdot \vec{S}_1)^2 - \right. \\ & \quad \frac{7}{3} \hat{n} \cdot \vec{v}_2 \vec{a}_1 \cdot \vec{v}_2 (\hat{n} \cdot \vec{S}_1)^2 - \hat{n} \cdot \vec{v}_2 \vec{v}_1 \cdot \vec{a}_1 (\hat{n} \cdot \vec{S}_1)^2 + 3 \hat{n} \cdot \vec{a}_1 \vec{v}_1 \cdot \vec{v}_2 (\hat{n} \cdot \vec{S}_1)^2 + \frac{1}{3} \hat{n} \cdot \vec{a}_1 \vec{v}_2 \cdot \vec{v}_2 (\hat{n} \cdot \vec{S}_1)^2 + \\ & \quad 4 \hat{n} \cdot \vec{S}_1 \hat{n} \cdot \vec{v}_1 (\hat{n} \cdot \vec{v}_2)^2 \hat{n} \cdot \vec{S}_1 - 12 \hat{n} \cdot \vec{S}_1 (\hat{n} \cdot \vec{v}_1)^2 \hat{n} \cdot \vec{v}_2 \hat{n} \cdot \vec{S}_1 + \frac{1}{3} (\hat{n} \cdot \vec{v}_2)^2 \vec{S}_1 \cdot \vec{v}_1 \hat{n} \cdot \vec{S}_1 + \\ & \quad 2 \hat{n} \cdot \vec{v}_1 \hat{n} \cdot \vec{v}_2 \vec{S}_1 \cdot \vec{v}_1 \hat{n} \cdot \vec{S}_1 + 4 (\hat{n} \cdot \vec{v}_1)^2 \vec{S}_1 \cdot \vec{v}_2 \hat{n} \cdot \vec{S}_1 - \frac{10}{3} \hat{n} \cdot \vec{v}_1 \hat{n} \cdot \vec{v}_2 \vec{S}_1 \cdot \vec{v}_2 \hat{n} \cdot \vec{S}_1 + \frac{2}{3} (\hat{n} \cdot \vec{v}_2)^2 \vec{S}_1 \cdot \vec{a}_1 \hat{n} \cdot \vec{S}_1 + \\ & \quad 2 \hat{n} \cdot \vec{a}_1 \hat{n} \cdot \vec{v}_2 \vec{S}_1 \cdot \vec{v}_1 \hat{n} \cdot \vec{S}_1 - \frac{5}{2} \vec{a}_1 \cdot \vec{v}_2 \vec{S}_1 \cdot \vec{v}_1 \hat{n} \cdot \vec{S}_1 + 2 \hat{n} \cdot \vec{a}_1 \hat{n} \cdot \vec{v}_1 \vec{S}_1 \cdot \vec{v}_2 \hat{n} \cdot \vec{S}_1 - \frac{2}{3} \hat{n} \cdot \vec{a}_1 \hat{n} \cdot \vec{v}_2 \vec{S}_1 \cdot \vec{v}_2 \hat{n} \cdot \vec{S}_1 + \\ & \quad \frac{2}{3} \vec{a}_1 \cdot \vec{v}_2 \vec{S}_1 \cdot \vec{v}_2 \hat{n} \cdot \vec{S}_1 + \frac{1}{2} \vec{S}_1 \cdot \vec{v}_2 \vec{v}_1 \cdot \vec{a}_1 \hat{n} \cdot \vec{S}_1 - \frac{1}{2} \vec{S}_1 \cdot \vec{v}_2 \vec{v}_1 \cdot \vec{v}_1 \hat{n} \cdot \vec{S}_1 + 12 \hat{n} \cdot \vec{S}_1 \hat{n} \cdot \vec{v}_1 \vec{v}_1 \cdot \vec{v}_2 \hat{n} \cdot \vec{S}_1 - \\ & \quad \frac{16}{3} \hat{n} \cdot \vec{S}_1 \hat{n} \cdot \vec{v}_2 \vec{v}_1 \cdot \vec{v}_2 \hat{n} \cdot \vec{S}_1 - \frac{5}{2} \vec{S}_1 \cdot \vec{v}_1 \vec{v}_1 \cdot \vec{v}_2 \hat{n} \cdot \vec{S}_1 + \frac{4}{3} \vec{S}_1 \cdot \vec{v}_2 \vec{v}_1 \cdot \vec{v}_2 \hat{n} \cdot \vec{S}_1 - \vec{S}_1 \cdot \vec{a}_1 \vec{v}_1 \cdot \vec{v}_2 \hat{n} \cdot \vec{S}_1 + \\ & \quad \frac{4}{3} \hat{n} \cdot \vec{S}_1 \hat{n} \cdot \vec{v}_1 \vec{v}_2 \cdot \vec{v}_2 \hat{n} \cdot \vec{S}_1 - \frac{5}{6} \vec{S}_1 \cdot \vec{v}_1 \vec{v}_2 \cdot \vec{v}_2 \hat{n} \cdot \vec{S}_1 - \frac{2}{3} \vec{S}_1 \cdot \vec{a}_1 \vec{v}_2 \cdot \vec{v}_2 \hat{n} \cdot \vec{S}_1 + \frac{1}{3} \hat{n} \cdot \vec{a}_1 (\vec{S}_1 \cdot \vec{v}_2)^2 + \\ & \quad \frac{10}{3} \hat{n} \cdot \vec{v}_1 (\hat{n} \cdot \vec{v}_2)^2 \vec{S}_1 \cdot \vec{S}_1 - 4 (\hat{n} \cdot \vec{v}_1)^2 \hat{n} \cdot \vec{v}_2 \vec{S}_1 \cdot \vec{S}_1 + \frac{1}{3} \hat{n} \cdot \vec{a}_1 (\hat{n} \cdot \vec{v}_2)^2 \vec{S}_1 \cdot \vec{S}_1 - 2 \hat{n} \cdot \vec{a}_1 \hat{n} \cdot \vec{v}_1 \hat{n} \cdot \vec{v}_2 \vec{S}_1 \cdot \vec{S}_1 + \\ & \quad \frac{1}{2} \hat{n} \cdot \vec{v}_1 \vec{a}_1 \cdot \vec{v}_2 \vec{S}_1 \cdot \vec{S}_1 + \frac{1}{3} \hat{n} \cdot \vec{v}_2 \vec{a}_1 \cdot \vec{v}_2 \vec{S}_1 \cdot \vec{S}_1 + \frac{1}{3} \hat{n} \cdot \vec{S}_1 (\hat{n} \cdot \vec{v}_2)^2 \vec{S}_1 \cdot \vec{v}_1 + 2 \hat{n} \cdot \vec{S}_1 \hat{n} \cdot \vec{v}_1 \hat{n} \cdot \vec{v}_2 \vec{S}_1 \cdot \vec{v}_1 -$$

$$\begin{aligned} & \frac{4}{3} \hat{n} \cdot \vec{S}_1 \vec{S}_1 \cdot \vec{v}_2 \vec{v}_1 \cdot \vec{v}_2 - \frac{1}{3} \hat{n} \cdot \vec{v}_1 \vec{S}_1 \cdot \vec{S}_1 \vec{v}_2 \cdot \vec{v}_2 - \frac{1}{3} \hat{n} \cdot \vec{a}_1 \vec{S}_1 \cdot \vec{S}_1 \vec{v}_2 \cdot \vec{v}_2 - \frac{5}{6} \hat{n} \cdot \vec{S}_1 \vec{S}_1 \cdot \vec{v}_1 \vec{v}_2 \cdot \vec{v}_2 \Big) + \\ & \frac{1}{\rho^4} \Big( 16 \left( \hat{n} \cdot \vec{S}_1 \right)^2 \hat{n} \cdot \vec{v}_2 \left( \hat{n} \cdot \vec{v}_1 \right)^3 + 4 \hat{n} \cdot \vec{v}_2 \vec{S}_1 \cdot \vec{S}_1 \left( \hat{n} \cdot \vec{v}_1 \right)^3 - 4 \hat{n} \cdot \vec{S}_1 \vec{S}_1 \cdot \vec{v}_2 \left( \hat{n} \cdot \vec{v}_1 \right)^3 - \\ & 8 \left( \hat{n} \cdot \vec{S}_1 \right)^2 \left( \hat{n} \cdot \vec{v}_2 \right)^2 \left( \hat{n} \cdot \vec{v}_1 \right)^2 - \frac{1}{3} \left( \vec{S}_1 \cdot \vec{v}_2 \right)^2 \left( \hat{n} \cdot \vec{v}_1 \right)^2 - 2 \left( \hat{n} \cdot \vec{v}_2 \right)^2 \vec{S}_1 \cdot \vec{S}_1 \left( \hat{n} \cdot \vec{v}_1 \right)^2 - \\ & 12 \hat{n} \cdot \vec{S}_1 \hat{n} \cdot \vec{v}_2 \vec{S}_1 \cdot \vec{v}_1 \left( \hat{n} \cdot \vec{v}_1 \right)^2 + 4 \hat{n} \cdot \vec{S}_1 \hat{n} \cdot \vec{v}_2 \vec{S}_1 \cdot \vec{v}_2 \left( \hat{n} \cdot \vec{v}_1 \right)^2 + 2 \vec{S}_1 \cdot \vec{v}_1 \vec{S}_1 \cdot \vec{v}_2 \left( \hat{n} \cdot \vec{v}_1 \right)^2 - \\ & 18 \left( \hat{n} \cdot \vec{S}_1 \right)^2 \vec{v}_1 \cdot \vec{v}_2 \left( \hat{n} \cdot \vec{v}_1 \right)^2 - 2 \vec{S}_1 \cdot \vec{S}_1 \vec{v}_1 \cdot \vec{v}_2 \left( \hat{n} \cdot \vec{v}_1 \right)^2 - 2 \left( \hat{n} \cdot \vec{S}_1 \right)^2 \vec{v}_2 \cdot \vec{v}_2 \left( \hat{n} \cdot \vec{v}_1 \right)^2 + \\ & \frac{1}{3} \vec{S}_1 \cdot \vec{S}_1 \vec{v}_2 \cdot \vec{v}_2 \left( \hat{n} \cdot \vec{v}_1 \right)^2 + 2 \hat{n} \cdot \vec{v}_2 \left( \vec{S}_1 \cdot \vec{v}_1 \right)^2 \hat{n} \cdot \vec{v}_1 + 4 \hat{n} \cdot \vec{S}_1 \left( \hat{n} \cdot \vec{v}_2 \right)^2 \vec{S}_1 \cdot \vec{v}_1 \hat{n} \cdot \vec{v}_1 - \\ & \frac{4}{3} \hat{n} \cdot \vec{v}_2 \vec{S}_1 \cdot \vec{v}_1 \vec{S}_1 \cdot \vec{v}_2 \hat{n} \cdot \vec{v}_1 - 2 \hat{n} \cdot \vec{v}_2 \vec{S}_1 \cdot \vec{S}_1 \vec{v}_1 \cdot \vec{v}_1 \hat{n} \cdot \vec{v}_1 + 16 \left( \hat{n} \cdot \vec{S}_1 \right)^2 \hat{n} \cdot \vec{v}_2 \vec{v}_1 \cdot \vec{v}_2 \hat{n} \cdot \vec{v}_1 + \\ & \frac{4}{3} \hat{n} \cdot \vec{v}_2 \vec{S}_1 \cdot \vec{S}_1 \vec{v}_1 \cdot \vec{v}_2 \hat{n} \cdot \vec{v}_1 + 12 \hat{n} \cdot \vec{S}_1 \vec{S}_1 \cdot \vec{v}_1 \vec{v}_1 \cdot \vec{v}_2 \hat{n} \cdot \vec{v}_1 - \frac{16}{3} \hat{n} \cdot \vec{S}_1 \vec{S}_1 \cdot \vec{v}_2 \vec{v}_1 \cdot \vec{v}_2 \hat{n} \cdot \vec{v}_1 + \\ & \frac{4}{3} \hat{n} \cdot \vec{S}_1 \vec{S}_1 \cdot \vec{v}_1 \vec{v}_2 \cdot \vec{v}_2 \hat{n} \cdot \vec{v}_1 - \frac{1}{3} \left( \hat{n} \cdot \vec{v}_2 \right)^2 \left( \vec{S}_1 \cdot \vec{v}_1 \right)^2 - \frac{4}{3} \left( \hat{n} \cdot \vec{S}_1 \right)^2 \left( \vec{v}_1 \cdot \vec{v}_2 \right)^2 - \frac{2}{3} \vec{S}_1 \cdot \vec{S}_1 \left( \vec{v}_1 \cdot \vec{v}_2 \right)^2 - \\ & 2 \left( \hat{n} \cdot \vec{S}_1 \right)^2 \left( \hat{n} \cdot \vec{v}_2 \right)^2 \vec{v}_1 \cdot \vec{v}_1 - \frac{1}{6} \left( \vec{S}_1 \cdot \vec{v}_2 \right)^2 \vec{v}_1 \cdot \vec{v}_1 + \frac{1}{3} \left( \hat{n} \cdot \vec{v}_2 \right)^2 \vec{S}_1 \cdot \vec{S}_1 \vec{v}_1 \cdot \vec{v}_1 + \frac{4}{3} \hat{n} \cdot \vec{S}_1 \hat{n} \cdot \vec{v}_2 \vec{S}_1 \cdot \vec{v}_2 \vec{v}_1 \cdot \vec{v}_1 - \\ & \frac{3}{2} \left( \vec{S}_1 \cdot \vec{v}_1 \right)^2 \vec{v}_1 \cdot \vec{v}_2 - \frac{16}{3} \hat{n} \cdot \vec{S}_1 \hat{n} \cdot \vec{v}_2 \vec{S}_1 \cdot \vec{v}_1 \vec{v}_1 \cdot \vec{v}_2 + \frac{4}{3} \vec{S}_1 \cdot \vec{v}_1 \vec{S}_1 \cdot \vec{v}_2 \vec{v}_1 \cdot \vec{v}_2 + 2 \left( \hat{n} \cdot \vec{S}_1 \right)^2 \vec{v}_1 \cdot \vec{v}_1 \vec{v}_1 \cdot \vec{v}_2 + \\ & \frac{1}{2} \vec{S}_1 \cdot \vec{S}_1 \vec{v}_1 \cdot \vec{v}_1 \vec{v}_1 \cdot \vec{v}_2 - \frac{1}{6} \left( \vec{S}_1 \cdot \vec{v}_1 \right)^2 \vec{v}_2 \cdot \vec{v}_2 + \frac{4}{3} \left( \hat{n} \cdot \vec{S}_1 \right)^2 \vec{v}_1 \cdot \vec{v}_1 \vec{v}_2 \cdot \vec{v}_2 - \frac{1}{3} \vec{S}_1 \cdot \vec{S}_1 \vec{v}_1 \cdot \vec{v}_1 \vec{v}_2 \cdot \vec{v}_2 \Big) \Big) m_2^2 C_{\text{ES}^2} \Big\} \end{aligned}$$

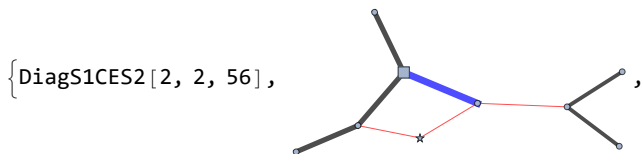

$$G^2 \left( \frac{1}{r} \left( -2 \hat{n} \cdot \vec{S}_1 \hat{n} \cdot \vec{S}_1 \hat{n} \cdot \vec{v}_1 - \frac{2}{3} \hat{n} \cdot \vec{S}_1 \hat{n} \cdot \vec{S}_1 \hat{n} \cdot \vec{v}_1 - 5 \vec{S}_1 \cdot \vec{S}_1 \hat{n} \cdot \vec{v}_1 - \right. \right. \\ \left. \frac{5}{3} \vec{S}_1 \cdot \vec{S}_1 \hat{n} \cdot \vec{v}_1 + \frac{5}{2} \hat{n} \cdot \vec{S}_1 \vec{S}_1 \cdot \vec{v}_1 + \frac{5}{2} \hat{n} \cdot \vec{S}_1 \vec{S}_1 \cdot \vec{v}_1 + \frac{5}{6} \hat{n} \cdot \vec{S}_1 \vec{S}_1 \cdot \vec{v}_1 + \frac{5}{6} \hat{n} \cdot \vec{S}_1 \vec{S}_1 \cdot \vec{v}_1 \right) + \\ \frac{1}{r^2} \left( 2 \left( \hat{n} \cdot \vec{v}_1 \right)^2 \left( \hat{n} \cdot \vec{S}_1 \right)^2 - \frac{8}{3} \hat{n} \cdot \vec{v}_1 \hat{n} \cdot \vec{v}_2 \left( \hat{n} \cdot \vec{S}_1 \right)^2 - \frac{3}{2} \vec{v}_1 \cdot \vec{v}_1 \left( \hat{n} \cdot \vec{S}_1 \right)^2 + \frac{2}{3} \vec{v}_1 \cdot \vec{v}_2 \left( \hat{n} \cdot \vec{S}_1 \right)^2 + \right. \\ \left. 2 \hat{n} \cdot \vec{a}_1 \hat{n} \cdot \vec{S}_1 \hat{n} \cdot \vec{v}_1 \hat{n} \cdot \vec{S}_1 - 3 \hat{n} \cdot \vec{v}_1 \vec{S}_1 \cdot \vec{v}_1 \hat{n} \cdot \vec{S}_1 + \frac{10}{3} \hat{n} \cdot \vec{v}_2 \vec{S}_1 \cdot \vec{v}_1 \hat{n} \cdot \vec{S}_1 + \frac{4}{3} \hat{n} \cdot \vec{v}_1 \vec{S}_1 \cdot \vec{v}_2 \hat{n} \cdot \vec{S}_1 - \right. \\ \frac{1}{4} \hat{n} \cdot \vec{v}_1 \vec{S}_1 \cdot \vec{a}_1 \hat{n} \cdot \vec{S}_1 - \frac{1}{4} \hat{n} \cdot \vec{a}_1 \vec{S}_1 \cdot \vec{v}_1 \hat{n} \cdot \vec{S}_1 - 4 \hat{n} \cdot \vec{S}_1 \vec{v}_1 \cdot \vec{a}_1 \hat{n} \cdot \vec{S}_1 + 2 \hat{n} \cdot \vec{S}_1 \hat{n} \cdot \vec{S}_1 \left( \hat{n} \cdot \vec{v}_1 \right)^2 + \left( \vec{S}_1 \cdot \vec{v}_1 \right)^2 + \\ \frac{1}{3} \hat{n} \cdot \vec{a}_1 \left( \hat{n} \cdot \vec{S}_1 \right)^2 \hat{n} \cdot \vec{v}_1 - \frac{8}{3} \hat{n} \cdot \vec{S}_1 \hat{n} \cdot \vec{S}_1 \hat{n} \cdot \vec{v}_1 \hat{n} \cdot \vec{v}_2 + \left( \hat{n} \cdot \vec{v}_1 \right)^2 \vec{S}_1 \cdot \vec{S}_1 - \frac{10}{3} \hat{n} \cdot \vec{v}_1 \hat{n} \cdot \vec{v}_2 \vec{S}_1 \cdot \vec{S}_1 - \\ \frac{1}{4} \hat{n} \cdot \vec{S}_1 \hat{n} \cdot \vec{v}_1 \vec{S}_1 \cdot \vec{a}_1 - \frac{1}{4} \hat{n} \cdot \vec{a}_1 \hat{n} \cdot \vec{S}_1 \vec{S}_1 \cdot \vec{v}_1 - \frac{5}{3} \vec{S}_1 \cdot \vec{v}_1 \vec{S}_1 \cdot \vec{v}_2 - \frac{3}{2} \hat{n} \cdot \vec{S}_1 \hat{n} \cdot \vec{v}_1 \vec{S}_1 \cdot \vec{v}_1 + \\ \frac{5}{3} \hat{n} \cdot \vec{S}_1 \hat{n} \cdot \vec{v}_2 \vec{S}_1 \cdot \vec{v}_1 + \frac{2}{3} \hat{n} \cdot \vec{S}_1 \hat{n} \cdot \vec{v}_1 \vec{S}_1 \cdot \vec{v}_2 - \frac{1}{6} \hat{n} \cdot \vec{S}_1 \hat{n} \cdot \vec{v}_1 \vec{S}_1 \cdot \vec{a}_1 - 2 \hat{n} \cdot \vec{a}_1 \hat{n} \cdot \vec{v}_1 \vec{S}_1 \cdot \vec{S}_1 + \left( \hat{n} \cdot \vec{v}_1 \right)^2 \vec{S}_1 \cdot \vec{S}_1 - \\ \frac{10}{3} \hat{n} \cdot \vec{v}_1 \hat{n} \cdot \vec{v}_2 \vec{S}_1 \cdot \vec{S}_1 - \frac{5}{6} \hat{n} \cdot \vec{a}_1 \hat{n} \cdot \vec{v}_1 \vec{S}_1 \cdot \vec{S}_1 + \frac{1}{3} \hat{n} \cdot \vec{a}_1 \hat{n} \cdot \vec{S}_1 \vec{S}_1 \cdot \vec{v}_1 - \frac{3}{2} \hat{n} \cdot \vec{S}_1 \hat{n} \cdot \vec{v}_1 \vec{S}_1 \cdot \vec{v}_1 + \\ \frac{5}{3} \hat{n} \cdot \vec{S}_1 \hat{n} \cdot \vec{v}_2 \vec{S}_1 \cdot \vec{v}_1 + \frac{2}{3} \vec{S}_1 \cdot \vec{v}_1 \vec{S}_1 \cdot \vec{v}_1 - \frac{5}{6} \vec{S}_1 \cdot \vec{v}_2 \vec{S}_1 \cdot \vec{v}_1 - \frac{1}{6} \vec{S}_1 \cdot \vec{a}_1 \vec{S}_1 \cdot \vec{v}_1 + \frac{2}{3} \hat{n} \cdot \vec{S}_1 \hat{n} \cdot \vec{v}_1 \vec{S}_1 \cdot \vec{v}_2 - \\ \frac{5}{6} \vec{S}_1 \cdot \vec{v}_1 \vec{S}_1 \cdot \vec{v}_2 - \frac{13}{12} \left( \hat{n} \cdot \vec{S}_1 \right)^2 \vec{v}_1 \cdot \vec{a}_1 + \frac{5}{12} \vec{S}_1 \cdot \vec{S}_1 \vec{v}_1 \cdot \vec{a}_1 + \vec{S}_1 \cdot \vec{S}_1 \vec{v}_1 \cdot \vec{a}_1 - \frac{3}{2} \hat{n} \cdot \vec{S}_1 \hat{n} \cdot \vec{S}_1 \vec{v}_1 \cdot \vec{v}_1 - \\ \left. \frac{1}{2} \vec{S}_1 \cdot \vec{S}_1 \vec{v}_1 \cdot \vec{v}_1 - \frac{1}{2} \vec{S}_1 \cdot \vec{S}_1 \vec{v}_1 \cdot \vec{v}_1 + \frac{2}{3} \hat{n} \cdot \vec{S}_1 \hat{n} \cdot \vec{S}_1 \vec{v}_1 \cdot \vec{v}_2 + \frac{5}{3} \vec{S}_1 \cdot \vec{S}_1 \vec{v}_1 \cdot \vec{v}_2 + \frac{5}{3} \vec{S}_1 \cdot \vec{S}_1 \vec{v}_1 \cdot \vec{v}_2 \right) + \frac{1}{r^3}$$

$$\begin{aligned}
& \left( -6 \hat{n} \cdot \vec{S}_1 \hat{n} \cdot \vec{S}_1 (\hat{n} \cdot \vec{v}_1)^3 - \vec{S}_1 \cdot \vec{S}_1 (\hat{n} \cdot \vec{v}_1)^3 - 3 \hat{n} \cdot \vec{a}_1 (\hat{n} \cdot \vec{S}_1)^2 (\hat{n} \cdot \vec{v}_1)^2 + 8 \hat{n} \cdot \vec{S}_1 \hat{n} \cdot \vec{S}_1 \hat{n} \cdot \vec{v}_2 (\hat{n} \cdot \vec{v}_1)^2 + \right. \\
& \frac{5}{2} \hat{n} \cdot \vec{S}_1 \vec{S}_1 \cdot \vec{v}_1 (\hat{n} \cdot \vec{v}_1)^2 - \frac{4}{3} \hat{n} \cdot \vec{S}_1 \vec{S}_1 \cdot \vec{v}_2 (\hat{n} \cdot \vec{v}_1)^2 - \frac{4}{3} \hat{n} \cdot \vec{v}_2 \vec{S}_1 \cdot \vec{S}_1 (\hat{n} \cdot \vec{v}_1)^2 + 2 \hat{n} \cdot \vec{a}_1 \vec{S}_1 \cdot \vec{S}_1 (\hat{n} \cdot \vec{v}_1)^2 + \\
& \frac{5}{2} \hat{n} \cdot \vec{S}_1 \vec{S}_1 \cdot \vec{v}_1 (\hat{n} \cdot \vec{v}_1)^2 - \frac{4}{3} \hat{n} \cdot \vec{S}_1 \vec{S}_1 \cdot \vec{v}_2 (\hat{n} \cdot \vec{v}_1)^2 + 2 \hat{n} \cdot \vec{a}_1 (\hat{n} \cdot \vec{S}_1)^2 \hat{n} \cdot \vec{v}_2 \hat{n} \cdot \vec{v}_1 - \\
& \frac{8}{3} \hat{n} \cdot \vec{S}_1 \hat{n} \cdot \vec{v}_2 \vec{S}_1 \cdot \vec{v}_1 \hat{n} \cdot \vec{v}_1 - \frac{1}{3} (\hat{n} \cdot \vec{S}_1)^2 \vec{a}_1 \cdot \vec{v}_2 \hat{n} \cdot \vec{v}_1 - \frac{2}{3} \hat{n} \cdot \vec{S}_1 \hat{n} \cdot \vec{v}_2 \vec{S}_1 \cdot \vec{a}_1 \hat{n} \cdot \vec{v}_1 - \\
& \frac{10}{3} \hat{n} \cdot \vec{a}_1 \hat{n} \cdot \vec{v}_2 \vec{S}_1 \cdot \vec{S}_1 \hat{n} \cdot \vec{v}_1 + \frac{5}{6} \vec{a}_1 \cdot \vec{v}_2 \vec{S}_1 \cdot \vec{S}_1 \hat{n} \cdot \vec{v}_1 - \hat{n} \cdot \vec{a}_1 \hat{n} \cdot \vec{S}_1 \vec{S}_1 \cdot \vec{v}_1 \hat{n} \cdot \vec{v}_1 - \\
& \frac{8}{3} \hat{n} \cdot \vec{S}_1 \hat{n} \cdot \vec{v}_2 \vec{S}_1 \cdot \vec{v}_1 \hat{n} \cdot \vec{v}_1 + \frac{2}{3} \vec{S}_1 \cdot \vec{v}_2 \vec{S}_1 \cdot \vec{v}_1 \hat{n} \cdot \vec{v}_1 + \vec{S}_1 \cdot \vec{a}_1 \vec{S}_1 \cdot \vec{v}_1 \hat{n} \cdot \vec{v}_1 - \frac{2}{3} \hat{n} \cdot \vec{a}_1 \hat{n} \cdot \vec{S}_1 \vec{S}_1 \cdot \vec{v}_2 \hat{n} \cdot \vec{v}_1 + \\
& \frac{2}{3} \vec{S}_1 \cdot \vec{v}_1 \vec{S}_1 \cdot \vec{v}_2 \hat{n} \cdot \vec{v}_1 + \frac{1}{6} \vec{S}_1 \cdot \vec{a}_1 \vec{S}_1 \cdot \vec{v}_2 \hat{n} \cdot \vec{v}_1 + \frac{11}{2} (\hat{n} \cdot \vec{S}_1)^2 \vec{v}_1 \cdot \vec{a}_1 \hat{n} \cdot \vec{v}_1 - \frac{3}{2} \vec{S}_1 \cdot \vec{S}_1 \vec{v}_1 \cdot \vec{a}_1 \hat{n} \cdot \vec{v}_1 + \\
& 10 \hat{n} \cdot \vec{S}_1 \hat{n} \cdot \vec{S}_1 \vec{v}_1 \cdot \vec{v}_1 \hat{n} \cdot \vec{v}_1 - 2 \vec{S}_1 \cdot \vec{S}_1 \vec{v}_1 \cdot \vec{v}_1 \hat{n} \cdot \vec{v}_1 - \frac{8}{3} \hat{n} \cdot \vec{S}_1 \hat{n} \cdot \vec{S}_1 \vec{v}_1 \cdot \vec{v}_2 \hat{n} \cdot \vec{v}_1 + \frac{2}{3} \vec{S}_1 \cdot \vec{S}_1 \vec{v}_1 \cdot \vec{v}_2 \hat{n} \cdot \vec{v}_1 + \\
& \hat{n} \cdot \vec{a}_1 (\vec{S}_1 \cdot \vec{v}_1)^2 + \frac{4}{3} \hat{n} \cdot \vec{a}_1 \hat{n} \cdot \vec{S}_1 \hat{n} \cdot \vec{v}_2 \vec{S}_1 \cdot \vec{v}_1 + \frac{2}{3} \hat{n} \cdot \vec{v}_2 \vec{S}_1 \cdot \vec{v}_1 \vec{S}_1 \cdot \vec{v}_1 - \frac{1}{3} \hat{n} \cdot \vec{S}_1 \vec{a}_1 \cdot \vec{v}_2 \vec{S}_1 \cdot \vec{v}_1 - \\
& \frac{1}{3} \hat{n} \cdot \vec{v}_2 \vec{S}_1 \cdot \vec{a}_1 \vec{S}_1 \cdot \vec{v}_1 - \frac{1}{3} \hat{n} \cdot \vec{a}_1 \vec{S}_1 \cdot \vec{v}_1 \vec{S}_1 \cdot \vec{v}_2 - \frac{13}{3} (\hat{n} \cdot \vec{S}_1)^2 \hat{n} \cdot \vec{v}_2 \vec{v}_1 \cdot \vec{a}_1 + \frac{5}{6} \hat{n} \cdot \vec{v}_2 \vec{S}_1 \cdot \vec{S}_1 \vec{v}_1 \cdot \vec{a}_1 - \\
& 2 \hat{n} \cdot \vec{S}_1 \vec{S}_1 \cdot \vec{v}_1 \vec{v}_1 \cdot \vec{a}_1 + \frac{13}{6} \hat{n} \cdot \vec{S}_1 \vec{S}_1 \cdot \vec{v}_2 \vec{v}_1 \cdot \vec{a}_1 + \frac{5}{2} \hat{n} \cdot \vec{a}_1 (\hat{n} \cdot \vec{S}_1)^2 \vec{v}_1 \cdot \vec{v}_1 - \frac{22}{3} \hat{n} \cdot \vec{S}_1 \hat{n} \cdot \vec{S}_1 \hat{n} \cdot \vec{v}_2 \vec{v}_1 \cdot \vec{v}_1 - \\
& 2 \hat{n} \cdot \vec{S}_1 \vec{S}_1 \cdot \vec{v}_1 \vec{v}_1 \cdot \vec{v}_1 + \frac{11}{6} \hat{n} \cdot \vec{S}_1 \vec{S}_1 \cdot \vec{v}_2 \vec{v}_1 \cdot \vec{v}_1 + \frac{1}{3} \hat{n} \cdot \vec{v}_2 \vec{S}_1 \cdot \vec{S}_1 \vec{v}_1 \cdot \vec{v}_1 - \hat{n} \cdot \vec{S}_1 \vec{S}_1 \cdot \vec{a}_1 \vec{v}_1 \cdot \vec{v}_1 - \\
& \frac{3}{2} \hat{n} \cdot \vec{a}_1 \vec{S}_1 \cdot \vec{S}_1 \vec{v}_1 \cdot \vec{v}_1 - 2 \hat{n} \cdot \vec{S}_1 \vec{S}_1 \cdot \vec{v}_1 \vec{v}_1 \cdot \vec{v}_1 + \frac{11}{6} \hat{n} \cdot \vec{S}_1 \vec{S}_1 \cdot \vec{v}_2 \vec{v}_1 \cdot \vec{v}_1 - \frac{1}{3} \hat{n} \cdot \vec{a}_1 (\hat{n} \cdot \vec{S}_1)^2 \vec{v}_1 \cdot \vec{v}_2 + \\
& \frac{2}{3} \hat{n} \cdot \vec{S}_1 \vec{S}_1 \cdot \vec{v}_1 \vec{v}_1 \cdot \vec{v}_2 + \frac{1}{6} \hat{n} \cdot \vec{S}_1 \vec{S}_1 \cdot \vec{a}_1 \vec{v}_1 \cdot \vec{v}_2 + \frac{5}{6} \hat{n} \cdot \vec{a}_1 \vec{S}_1 \cdot \vec{S}_1 \vec{v}_1 \cdot \vec{v}_2 + \frac{2}{3} \hat{n} \cdot \vec{S}_1 \vec{S}_1 \cdot \vec{v}_1 \vec{v}_1 \cdot \vec{v}_2 \Big) + \frac{1}{r^4} \\
& \left( 5 (\hat{n} \cdot \vec{S}_1)^2 (\hat{n} \cdot \vec{v}_1)^4 - \frac{7}{4} \vec{S}_1 \cdot \vec{S}_1 (\hat{n} \cdot \vec{v}_1)^4 - 8 (\hat{n} \cdot \vec{S}_1)^2 \hat{n} \cdot \vec{v}_2 (\hat{n} \cdot \vec{v}_1)^3 + 4 \hat{n} \cdot \vec{v}_2 \vec{S}_1 \cdot \vec{S}_1 (\hat{n} \cdot \vec{v}_1)^3 + \right. \\
& \frac{1}{4} \hat{n} \cdot \vec{S}_1 \vec{S}_1 \cdot \vec{v}_1 (\hat{n} \cdot \vec{v}_1)^3 + 2 \hat{n} \cdot \vec{S}_1 \vec{S}_1 \cdot \vec{v}_2 (\hat{n} \cdot \vec{v}_1)^3 - \frac{5}{4} (\vec{S}_1 \cdot \vec{v}_1)^2 (\hat{n} \cdot \vec{v}_1)^2 - 6 \hat{n} \cdot \vec{S}_1 \hat{n} \cdot \vec{v}_2 \vec{S}_1 \cdot \vec{v}_1 (\hat{n} \cdot \vec{v}_1)^2 + \\
& \vec{S}_1 \cdot \vec{v}_1 \vec{S}_1 \cdot \vec{v}_2 (\hat{n} \cdot \vec{v}_1)^2 - \frac{105}{8} (\hat{n} \cdot \vec{S}_1)^2 \vec{v}_1 \cdot \vec{v}_1 (\hat{n} \cdot \vec{v}_1)^2 + \frac{27}{8} \vec{S}_1 \cdot \vec{S}_1 \vec{v}_1 \cdot \vec{v}_1 (\hat{n} \cdot \vec{v}_1)^2 + \\
& 3 (\hat{n} \cdot \vec{S}_1)^2 \vec{v}_1 \cdot \vec{v}_2 (\hat{n} \cdot \vec{v}_1)^2 - 2 \vec{S}_1 \cdot \vec{S}_1 \vec{v}_1 \cdot \vec{v}_2 (\hat{n} \cdot \vec{v}_1)^2 + 4 \hat{n} \cdot \vec{v}_2 (\vec{S}_1 \cdot \vec{v}_1)^2 \hat{n} \cdot \vec{v}_1 + 18 (\hat{n} \cdot \vec{S}_1)^2 \hat{n} \cdot \vec{v}_2 \vec{v}_1 \cdot \vec{v}_1 \hat{n} \cdot \vec{v}_1 - \\
& 4 \hat{n} \cdot \vec{v}_2 \vec{S}_1 \cdot \vec{S}_1 \vec{v}_1 \cdot \vec{v}_1 \hat{n} \cdot \vec{v}_1 + \frac{17}{4} \hat{n} \cdot \vec{S}_1 \vec{S}_1 \cdot \vec{v}_1 \vec{v}_1 \cdot \vec{v}_1 \hat{n} \cdot \vec{v}_1 - 6 \hat{n} \cdot \vec{S}_1 \vec{S}_1 \cdot \vec{v}_2 \vec{v}_1 \cdot \vec{v}_1 \hat{n} \cdot \vec{v}_1 + \\
& 2 \hat{n} \cdot \vec{S}_1 \vec{S}_1 \cdot \vec{v}_1 \vec{v}_1 \cdot \vec{v}_2 \hat{n} \cdot \vec{v}_1 + \frac{15}{8} (\hat{n} \cdot \vec{S}_1)^2 (\vec{v}_1 \cdot \vec{v}_1)^2 - \frac{5}{8} \vec{S}_1 \cdot \vec{S}_1 (\vec{v}_1 \cdot \vec{v}_1)^2 - 4 \hat{n} \cdot \vec{S}_1 \hat{n} \cdot \vec{v}_2 \vec{S}_1 \cdot \vec{v}_1 \vec{v}_1 \cdot \vec{v}_1 + \\
& \left. \vec{S}_1 \cdot \vec{v}_1 \vec{S}_1 \cdot \vec{v}_2 \vec{v}_1 \cdot \vec{v}_1 - (\vec{S}_1 \cdot \vec{v}_1)^2 \vec{v}_1 \cdot \vec{v}_2 - 3 (\hat{n} \cdot \vec{S}_1)^2 \vec{v}_1 \cdot \vec{v}_1 \vec{v}_1 \cdot \vec{v}_2 + \vec{S}_1 \cdot \vec{S}_1 \vec{v}_1 \cdot \vec{v}_1 \vec{v}_1 \cdot \vec{v}_2 \right) \Big) m_2 C_{ES^2 1} \}
\end{aligned}$$

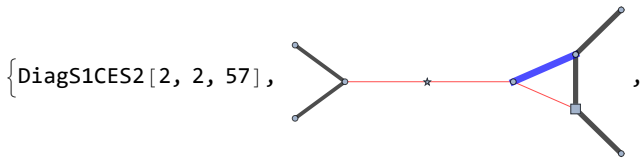

$$\begin{aligned}
& G^2 \left( \frac{1}{r^3} \left( 20 \hat{n} \cdot \vec{a}_1 \hat{n} \cdot \vec{v}_1 \hat{n} \cdot \vec{v}_2 (\hat{n} \cdot \vec{S}_1)^2 - \frac{10}{3} \hat{n} \cdot \vec{v}_1 \vec{a}_1 \cdot \vec{v}_2 (\hat{n} \cdot \vec{S}_1)^2 - \frac{10}{3} \hat{n} \cdot \vec{v}_2 \vec{v}_1 \cdot \vec{a}_1 (\hat{n} \cdot \vec{S}_1)^2 - \right. \right. \\
& \frac{10}{3} \hat{n} \cdot \vec{a}_1 \vec{v}_1 \cdot \vec{v}_2 (\hat{n} \cdot \vec{S}_1)^2 + 20 \hat{n} \cdot \vec{S}_1 (\hat{n} \cdot \vec{v}_1)^2 \hat{n} \cdot \vec{v}_2 \hat{n} \cdot \vec{S}_1 - \frac{14}{3} \hat{n} \cdot \vec{v}_1 \hat{n} \cdot \vec{v}_2 \vec{S}_1 \cdot \vec{v}_1 \hat{n} \cdot \vec{S}_1 - \\
& \left. \frac{10}{3} (\hat{n} \cdot \vec{v}_1)^2 \vec{S}_1 \cdot \vec{v}_2 \hat{n} \cdot \vec{S}_1 - \frac{14}{3} \hat{n} \cdot \vec{v}_1 \hat{n} \cdot \vec{v}_2 \vec{S}_1 \cdot \vec{a}_1 \hat{n} \cdot \vec{S}_1 - \frac{14}{3} \hat{n} \cdot \vec{a}_1 \hat{n} \cdot \vec{v}_2 \vec{S}_1 \cdot \vec{v}_1 \hat{n} \cdot \vec{S}_1 + \frac{7}{6} \vec{a}_1 \cdot \vec{v}_2 \vec{S}_1 \cdot \vec{v}_1 \hat{n} \cdot \vec{S}_1 - \right.
\end{aligned}$$

$$\begin{aligned}
& \frac{20}{3} \hat{n} \cdot \vec{a}_1 \hat{n} \cdot \vec{v}_1 \vec{S}_1 \cdot \vec{v}_2 \hat{n} \cdot \vec{S}_1 + \frac{5}{3} \vec{S}_1 \cdot \vec{v}_2 \vec{v}_1 \cdot \vec{a}_1 \hat{n} \cdot \vec{S}_1 - \frac{10}{3} \hat{n} \cdot \vec{S}_1 \hat{n} \cdot \vec{v}_2 \vec{v}_1 \cdot \vec{v}_1 \hat{n} \cdot \vec{S}_1 + \frac{5}{6} \vec{S}_1 \cdot \vec{v}_2 \vec{v}_1 \cdot \vec{v}_1 \hat{n} \cdot \vec{S}_1 - \\
& \frac{20}{3} \hat{n} \cdot \vec{S}_1 \hat{n} \cdot \vec{v}_1 \vec{v}_1 \cdot \vec{v}_2 \hat{n} \cdot \vec{S}_1 + \frac{7}{6} \vec{S}_1 \cdot \vec{v}_1 \vec{v}_1 \cdot \vec{v}_2 \hat{n} \cdot \vec{S}_1 + \frac{7}{6} \vec{S}_1 \cdot \vec{a}_1 \vec{v}_1 \cdot \vec{v}_2 \hat{n} \cdot \vec{S}_1 - \frac{4}{3} (\hat{n} \cdot \vec{v}_1)^2 \hat{n} \cdot \vec{v}_2 \vec{S}_1 \cdot \vec{S}_1 - \\
& \frac{4}{3} \hat{n} \cdot \vec{a}_1 \hat{n} \cdot \vec{v}_1 \hat{n} \cdot \vec{v}_2 \vec{S}_1 \cdot \vec{S}_1 + \frac{1}{3} \hat{n} \cdot \vec{v}_1 \vec{a}_1 \cdot \vec{v}_2 \vec{S}_1 \cdot \vec{S}_1 - \frac{14}{3} \hat{n} \cdot \vec{S}_1 \hat{n} \cdot \vec{v}_1 \hat{n} \cdot \vec{v}_2 \vec{S}_1 \cdot \vec{v}_1 + \frac{2}{3} \hat{n} \cdot \vec{v}_2 \vec{S}_1 \cdot \vec{v}_1 \vec{S}_1 \cdot \vec{v}_1 + \\
& \frac{7}{6} \hat{n} \cdot \vec{v}_1 \vec{S}_1 \cdot \vec{v}_2 \vec{S}_1 \cdot \vec{v}_1 + \frac{2}{3} \hat{n} \cdot \vec{v}_2 \vec{S}_1 \cdot \vec{a}_1 \vec{S}_1 \cdot \vec{v}_1 - \frac{10}{3} \hat{n} \cdot \vec{S}_1 (\hat{n} \cdot \vec{v}_1)^2 \vec{S}_1 \cdot \vec{v}_2 + \frac{7}{6} \hat{n} \cdot \vec{v}_1 \vec{S}_1 \cdot \vec{v}_1 \vec{S}_1 \cdot \vec{v}_2 + \\
& \frac{7}{6} \hat{n} \cdot \vec{v}_1 \vec{S}_1 \cdot \vec{a}_1 \vec{S}_1 \cdot \vec{v}_2 + \frac{7}{6} \hat{n} \cdot \vec{a}_1 \vec{S}_1 \cdot \vec{v}_1 \vec{S}_1 \cdot \vec{v}_2 + \frac{1}{3} \hat{n} \cdot \vec{v}_2 \vec{S}_1 \cdot \vec{S}_1 \vec{v}_1 \cdot \vec{a}_1 + \frac{1}{3} \hat{n} \cdot \vec{v}_2 \vec{S}_1 \cdot \vec{S}_1 \vec{v}_1 \cdot \vec{v}_1 + \\
& \frac{5}{6} \hat{n} \cdot \vec{S}_1 \vec{S}_1 \cdot \vec{v}_2 \vec{v}_1 \cdot \vec{v}_1 + \frac{2}{3} \hat{n} \cdot \vec{v}_1 \vec{S}_1 \cdot \vec{S}_1 \vec{v}_1 \cdot \vec{v}_2 + \frac{1}{3} \hat{n} \cdot \vec{a}_1 \vec{S}_1 \cdot \vec{S}_1 \vec{v}_1 \cdot \vec{v}_2 + \frac{7}{6} \hat{n} \cdot \vec{S}_1 \vec{S}_1 \cdot \vec{v}_1 \vec{v}_1 \cdot \vec{v}_2 \Big) + \\
& \frac{1}{r^4} \left( -80 (\hat{n} \cdot \vec{S}_1)^2 \hat{n} \cdot \vec{v}_2 (\hat{n} \cdot \vec{v}_1)^3 + 4 \hat{n} \cdot \vec{v}_2 \vec{S}_1 \cdot \vec{S}_1 (\hat{n} \cdot \vec{v}_1)^3 + 20 \hat{n} \cdot \vec{S}_1 \vec{S}_1 \cdot \vec{v}_2 (\hat{n} \cdot \vec{v}_1)^3 + \right. \\
& 48 \hat{n} \cdot \vec{S}_1 \hat{n} \cdot \vec{v}_2 \vec{S}_1 \cdot \vec{v}_1 (\hat{n} \cdot \vec{v}_1)^2 - 8 \vec{S}_1 \cdot \vec{v}_1 \vec{S}_1 \cdot \vec{v}_2 (\hat{n} \cdot \vec{v}_1)^2 + 30 (\hat{n} \cdot \vec{S}_1)^2 \vec{v}_1 \cdot \vec{v}_2 (\hat{n} \cdot \vec{v}_1)^2 - \\
& 2 \vec{S}_1 \cdot \vec{S}_1 \vec{v}_1 \cdot \vec{v}_2 (\hat{n} \cdot \vec{v}_1)^2 - 6 \hat{n} \cdot \vec{v}_2 (\vec{S}_1 \cdot \vec{v}_1)^2 \hat{n} \cdot \vec{v}_1 + 30 (\hat{n} \cdot \vec{S}_1)^2 \hat{n} \cdot \vec{v}_2 \vec{v}_1 \cdot \vec{v}_1 \hat{n} \cdot \vec{v}_1 - 2 \hat{n} \cdot \vec{v}_2 \vec{S}_1 \cdot \vec{S}_1 \vec{v}_1 \cdot \vec{v}_1 \hat{n} \cdot \vec{v}_1 - \\
& 10 \hat{n} \cdot \vec{S}_1 \vec{S}_1 \cdot \vec{v}_2 \vec{v}_1 \cdot \vec{v}_1 \hat{n} \cdot \vec{v}_1 - 16 \hat{n} \cdot \vec{S}_1 \vec{S}_1 \cdot \vec{v}_1 \vec{v}_1 \cdot \vec{v}_2 \hat{n} \cdot \vec{v}_1 - 8 \hat{n} \cdot \vec{S}_1 \hat{n} \cdot \vec{v}_2 \vec{S}_1 \cdot \vec{v}_1 \vec{v}_1 \cdot \vec{v}_1 + \\
& \left. 2 \vec{S}_1 \cdot \vec{v}_1 \vec{S}_1 \cdot \vec{v}_2 \vec{v}_1 \cdot \vec{v}_1 + \frac{3}{2} (\vec{S}_1 \cdot \vec{v}_1)^2 \vec{v}_1 \cdot \vec{v}_2 - 5 (\hat{n} \cdot \vec{S}_1)^2 \vec{v}_1 \cdot \vec{v}_1 \vec{v}_1 \cdot \vec{v}_2 + \frac{1}{2} \vec{S}_1 \cdot \vec{S}_1 \vec{v}_1 \cdot \vec{v}_1 \vec{v}_1 \cdot \vec{v}_2 \right) \Big) m_2 C_{ES^2 1} \Big\}
\end{aligned}$$

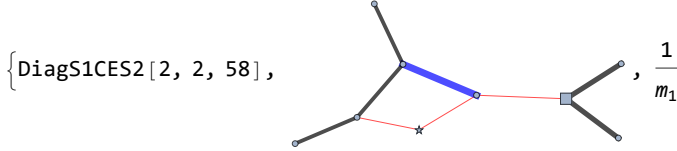

$$\begin{aligned}
& G^2 \left( \frac{1}{r^3} \left( 16 \hat{n} \cdot \vec{S}_1 \hat{n} \cdot \vec{S}_1 (\hat{n} \cdot \vec{v}_2)^3 + \frac{16}{3} \vec{S}_1 \cdot \vec{S}_1 (\hat{n} \cdot \vec{v}_2)^3 + 16 \hat{n} \cdot \vec{a}_2 (\hat{n} \cdot \vec{S}_1)^2 (\hat{n} \cdot \vec{v}_2)^2 - 8 \hat{n} \cdot \vec{S}_1 \vec{S}_1 \cdot \vec{v}_2 (\hat{n} \cdot \vec{v}_2)^2 - \right. \right. \\
& \frac{16}{3} \hat{n} \cdot \vec{S}_1 \vec{S}_1 \cdot \vec{a}_2 (\hat{n} \cdot \vec{v}_2)^2 + \frac{16}{3} \hat{n} \cdot \vec{a}_2 \vec{S}_1 \cdot \vec{S}_1 (\hat{n} \cdot \vec{v}_2)^2 - 8 \hat{n} \cdot \vec{S}_1 \vec{S}_1 \cdot \vec{v}_2 (\hat{n} \cdot \vec{v}_2)^2 - \frac{32}{3} \hat{n} \cdot \vec{a}_2 \hat{n} \cdot \vec{S}_1 \vec{S}_1 \cdot \vec{v}_2 \hat{n} \cdot \vec{v}_2 + \\
& 4 \vec{S}_1 \cdot \vec{v}_2 \vec{S}_1 \cdot \vec{v}_2 \hat{n} \cdot \vec{v}_2 + \frac{8}{3} \vec{S}_1 \cdot \vec{a}_2 \vec{S}_1 \cdot \vec{v}_2 \hat{n} \cdot \vec{v}_2 - \frac{28}{3} (\hat{n} \cdot \vec{S}_1)^2 \vec{v}_2 \cdot \vec{a}_2 \hat{n} \cdot \vec{v}_2 - \frac{8}{3} \vec{S}_1 \cdot \vec{S}_1 \vec{v}_2 \cdot \vec{a}_2 \hat{n} \cdot \vec{v}_2 - 16 \hat{n} \cdot \vec{S}_1 \hat{n} \cdot \vec{S}_1 \\
& \vec{v}_2 \cdot \vec{v}_2 \hat{n} \cdot \vec{v}_2 - 4 \vec{S}_1 \cdot \vec{S}_1 \vec{v}_2 \cdot \vec{v}_2 \hat{n} \cdot \vec{v}_2 + \frac{4}{3} \hat{n} \cdot \vec{a}_2 (\vec{S}_1 \cdot \vec{v}_2)^2 + \frac{14}{3} \hat{n} \cdot \vec{S}_1 \vec{S}_1 \cdot \vec{v}_2 \vec{v}_2 \cdot \vec{a}_2 - \frac{20}{3} \hat{n} \cdot \vec{a}_2 (\hat{n} \cdot \vec{S}_1)^2 \vec{v}_2 \cdot \vec{v}_2 + \\
& \left. 4 \hat{n} \cdot \vec{S}_1 \vec{S}_1 \cdot \vec{v}_2 \vec{v}_2 \cdot \vec{v}_2 + \frac{10}{3} \hat{n} \cdot \vec{S}_1 \vec{S}_1 \cdot \vec{a}_2 \vec{v}_2 \cdot \vec{v}_2 - \frac{4}{3} \hat{n} \cdot \vec{a}_2 \vec{S}_1 \cdot \vec{S}_1 \vec{v}_2 \cdot \vec{v}_2 + 4 \hat{n} \cdot \vec{S}_1 \vec{S}_1 \cdot \vec{v}_2 \vec{v}_2 \cdot \vec{v}_2 \right) + \frac{1}{r^4} \\
& \left( 16 (\hat{n} \cdot \vec{S}_1)^2 (\hat{n} \cdot \vec{v}_2)^4 + 4 \vec{S}_1 \cdot \vec{S}_1 (\hat{n} \cdot \vec{v}_2)^4 - 64 (\hat{n} \cdot \vec{S}_1)^2 \hat{n} \cdot \vec{v}_1 (\hat{n} \cdot \vec{v}_2)^3 - 16 \hat{n} \cdot \vec{v}_1 \vec{S}_1 \cdot \vec{S}_1 (\hat{n} \cdot \vec{v}_2)^3 + \right. \\
& 16 \hat{n} \cdot \vec{S}_1 \vec{S}_1 \cdot \vec{v}_1 (\hat{n} \cdot \vec{v}_2)^3 - 16 \hat{n} \cdot \vec{S}_1 \vec{S}_1 \cdot \vec{v}_2 (\hat{n} \cdot \vec{v}_2)^3 + 4 (\vec{S}_1 \cdot \vec{v}_2)^2 (\hat{n} \cdot \vec{v}_2)^2 + 48 \hat{n} \cdot \vec{S}_1 \hat{n} \cdot \vec{v}_1 \vec{S}_1 \cdot \vec{v}_2 (\hat{n} \cdot \vec{v}_2)^2 - \\
& 8 \vec{S}_1 \cdot \vec{v}_1 \vec{S}_1 \cdot \vec{v}_2 (\hat{n} \cdot \vec{v}_2)^2 + 24 (\hat{n} \cdot \vec{S}_1)^2 \vec{v}_1 \cdot \vec{v}_2 (\hat{n} \cdot \vec{v}_2)^2 + 8 \vec{S}_1 \cdot \vec{S}_1 \vec{v}_1 \cdot \vec{v}_2 (\hat{n} \cdot \vec{v}_2)^2 - \\
& 18 (\hat{n} \cdot \vec{S}_1)^2 \vec{v}_2 \cdot \vec{v}_2 (\hat{n} \cdot \vec{v}_2)^2 - 4 \vec{S}_1 \cdot \vec{S}_1 \vec{v}_2 \cdot \vec{v}_2 (\hat{n} \cdot \vec{v}_2)^2 - 8 \hat{n} \cdot \vec{v}_1 (\vec{S}_1 \cdot \vec{v}_2)^2 \hat{n} \cdot \vec{v}_2 - \\
& 16 \hat{n} \cdot \vec{S}_1 \vec{S}_1 \cdot \vec{v}_2 \vec{v}_1 \cdot \vec{v}_2 \hat{n} \cdot \vec{v}_2 + 48 (\hat{n} \cdot \vec{S}_1)^2 \hat{n} \cdot \vec{v}_1 \vec{v}_2 \cdot \vec{v}_2 \hat{n} \cdot \vec{v}_2 + 8 \hat{n} \cdot \vec{v}_1 \vec{S}_1 \cdot \vec{S}_1 \vec{v}_2 \cdot \vec{v}_2 \hat{n} \cdot \vec{v}_2 - \\
& 16 \hat{n} \cdot \vec{S}_1 \vec{S}_1 \cdot \vec{v}_1 \vec{v}_2 \cdot \vec{v}_2 \hat{n} \cdot \vec{v}_2 + 12 \hat{n} \cdot \vec{S}_1 \vec{S}_1 \cdot \vec{v}_2 \vec{v}_2 \cdot \vec{v}_2 \hat{n} \cdot \vec{v}_2 + 2 (\hat{n} \cdot \vec{S}_1)^2 (\vec{v}_2 \cdot \vec{v}_2)^2 + \\
& \frac{1}{2} \vec{S}_1 \cdot \vec{S}_1 (\vec{v}_2 \cdot \vec{v}_2)^2 + 2 (\vec{S}_1 \cdot \vec{v}_2)^2 \vec{v}_1 \cdot \vec{v}_2 - \frac{3}{2} (\vec{S}_1 \cdot \vec{v}_2)^2 \vec{v}_2 \cdot \vec{v}_2 - 16 \hat{n} \cdot \vec{S}_1 \hat{n} \cdot \vec{v}_1 \vec{S}_1 \cdot \vec{v}_2 \vec{v}_2 \cdot \vec{v}_2 + \\
& \left. 4 \vec{S}_1 \cdot \vec{v}_1 \vec{S}_1 \cdot \vec{v}_2 \vec{v}_2 \cdot \vec{v}_2 - 8 (\hat{n} \cdot \vec{S}_1)^2 \vec{v}_1 \cdot \vec{v}_2 \vec{v}_2 \cdot \vec{v}_2 - 2 \vec{S}_1 \cdot \vec{S}_1 \vec{v}_1 \cdot \vec{v}_2 \vec{v}_2 \cdot \vec{v}_2 \right) \Big) m_2^2 C_{ES^2 1} \Big\}
\end{aligned}$$

{DiagS1CES2[2, 2, 59],

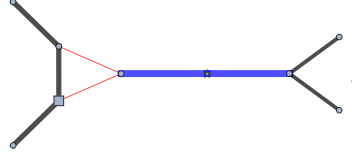

,

$$\begin{aligned}
 G^2 \left( \frac{1}{r^2} \left( -\frac{5}{6} \hat{n} \cdot \vec{S}_1 \hat{n} \cdot \vec{a}_2 \hat{n} \cdot \vec{S}_1 \hat{n} \cdot \vec{v}_2 + \frac{1}{3} \hat{n} \cdot \vec{S}_1 \vec{S}_1 \cdot \vec{a}_2 \hat{n} \cdot \vec{v}_2 - \frac{1}{6} \hat{n} \cdot \vec{a}_2 \vec{S}_1 \cdot \vec{S}_1 \hat{n} \cdot \vec{v}_2 + \frac{1}{3} \hat{n} \cdot \vec{S}_1 \vec{S}_1 \cdot \vec{a}_2 \hat{n} \cdot \vec{v}_2 + \frac{1}{3} \hat{n} \cdot \vec{a}_2 \hat{n} \cdot \vec{S}_1 \right. \right. \\
 \left. \left. \vec{S}_1 \cdot \vec{v}_2 - \frac{1}{6} \vec{S}_1 \cdot \vec{v}_2 \vec{S}_1 \cdot \vec{a}_2 + \frac{1}{3} \hat{n} \cdot \vec{S}_1 \hat{n} \cdot \vec{a}_2 \vec{S}_1 \cdot \vec{v}_2 - \frac{1}{6} \vec{S}_1 \cdot \vec{a}_2 \vec{S}_1 \cdot \vec{v}_2 + \frac{5}{6} \hat{n} \cdot \vec{S}_1 \hat{n} \cdot \vec{S}_1 \vec{v}_2 \cdot \vec{a}_2 - \frac{1}{6} \vec{S}_1 \cdot \vec{S}_1 \vec{v}_2 \cdot \vec{a}_2 \right) + \right. \\
 \left. \frac{1}{r^3} \left( -\frac{5}{2} \hat{n} \cdot \vec{S}_1 \hat{n} \cdot \vec{S}_1 (\hat{n} \cdot \vec{v}_2)^3 - \frac{1}{3} \vec{S}_1 \cdot \vec{S}_1 (\hat{n} \cdot \vec{v}_2)^3 + \frac{7}{4} \hat{n} \cdot \vec{S}_1 \vec{S}_1 \cdot \vec{v}_2 (\hat{n} \cdot \vec{v}_2)^2 + \frac{7}{4} \hat{n} \cdot \vec{S}_1 \vec{S}_1 \cdot \vec{v}_2 (\hat{n} \cdot \vec{v}_2)^2 + \right. \right. \\
 \left. \left. \frac{5}{2} \hat{n} \cdot \vec{a}_2 (\hat{n} \cdot \vec{S}_1)^2 \hat{n} \cdot \vec{v}_1 \hat{n} \cdot \vec{v}_2 - \frac{4}{3} \hat{n} \cdot \vec{S}_1 \hat{n} \cdot \vec{v}_1 \vec{S}_1 \cdot \vec{a}_2 \hat{n} \cdot \vec{v}_2 + \frac{1}{3} \hat{n} \cdot \vec{a}_2 \hat{n} \cdot \vec{v}_1 \vec{S}_1 \cdot \vec{S}_1 \hat{n} \cdot \vec{v}_2 - \right. \right. \\
 \left. \left. \frac{5}{6} \hat{n} \cdot \vec{a}_2 \hat{n} \cdot \vec{S}_1 \vec{S}_1 \cdot \vec{v}_1 \hat{n} \cdot \vec{v}_2 + \frac{1}{3} \vec{S}_1 \cdot \vec{a}_2 \vec{S}_1 \cdot \vec{v}_1 \hat{n} \cdot \vec{v}_2 - \vec{S}_1 \cdot \vec{v}_2 \vec{S}_1 \cdot \vec{v}_2 \hat{n} \cdot \vec{v}_2 - \frac{5}{12} (\hat{n} \cdot \vec{S}_1)^2 \vec{v}_1 \cdot \vec{a}_2 \hat{n} \cdot \vec{v}_2 - \right. \right. \\
 \left. \left. \frac{1}{12} \vec{S}_1 \cdot \vec{S}_1 \vec{v}_1 \cdot \vec{a}_2 \hat{n} \cdot \vec{v}_2 + \frac{5}{2} \hat{n} \cdot \vec{S}_1 \hat{n} \cdot \vec{S}_1 \vec{v}_2 \cdot \vec{v}_2 \hat{n} \cdot \vec{v}_2 - \frac{4}{3} \hat{n} \cdot \vec{a}_2 \hat{n} \cdot \vec{S}_1 \hat{n} \cdot \vec{v}_1 \vec{S}_1 \cdot \vec{v}_2 + \right. \right. \\
 \left. \left. \frac{1}{3} \hat{n} \cdot \vec{v}_1 \vec{S}_1 \cdot \vec{a}_2 \vec{S}_1 \cdot \vec{v}_2 + \frac{1}{3} \hat{n} \cdot \vec{a}_2 \vec{S}_1 \cdot \vec{v}_1 \vec{S}_1 \cdot \vec{v}_2 + \frac{1}{3} \hat{n} \cdot \vec{S}_1 \vec{S}_1 \cdot \vec{v}_2 \vec{v}_1 \cdot \vec{a}_2 - \frac{5}{12} \hat{n} \cdot \vec{a}_2 (\hat{n} \cdot \vec{S}_1)^2 \vec{v}_1 \cdot \vec{v}_2 + \right. \right. \\
 \left. \left. \frac{1}{3} \hat{n} \cdot \vec{S}_1 \vec{S}_1 \cdot \vec{a}_2 \vec{v}_1 \cdot \vec{v}_2 - \frac{1}{12} \hat{n} \cdot \vec{a}_2 \vec{S}_1 \cdot \vec{S}_1 \vec{v}_1 \cdot \vec{v}_2 - \frac{5}{3} (\hat{n} \cdot \vec{S}_1)^2 \hat{n} \cdot \vec{v}_1 \vec{v}_2 \cdot \vec{a}_2 + \frac{1}{6} \hat{n} \cdot \vec{v}_1 \vec{S}_1 \cdot \vec{S}_1 \vec{v}_2 \cdot \vec{a}_2 + \right. \right. \\
 \left. \left. \frac{5}{6} \hat{n} \cdot \vec{S}_1 \vec{S}_1 \cdot \vec{v}_1 \vec{v}_2 \cdot \vec{a}_2 - \frac{3}{4} \hat{n} \cdot \vec{S}_1 \vec{S}_1 \cdot \vec{v}_2 \vec{v}_2 \cdot \vec{v}_2 - \frac{3}{4} \hat{n} \cdot \vec{S}_1 \vec{S}_1 \cdot \vec{v}_2 \vec{v}_2 \cdot \vec{v}_2 \right) + \frac{1}{r^4} \right. \\
 \left. \left( 10 (\hat{n} \cdot \vec{S}_1)^2 \hat{n} \cdot \vec{v}_1 (\hat{n} \cdot \vec{v}_2)^3 + \hat{n} \cdot \vec{v}_1 \vec{S}_1 \cdot \vec{S}_1 (\hat{n} \cdot \vec{v}_2)^3 - \frac{5}{2} \hat{n} \cdot \vec{S}_1 \vec{S}_1 \cdot \vec{v}_1 (\hat{n} \cdot \vec{v}_2)^3 - \frac{21}{2} \hat{n} \cdot \vec{S}_1 \hat{n} \cdot \vec{v}_1 \vec{S}_1 \cdot \vec{v}_2 (\hat{n} \cdot \vec{v}_2)^2 + \right. \right. \\
 \left. \left. \frac{7}{4} \vec{S}_1 \cdot \vec{v}_1 \vec{S}_1 \cdot \vec{v}_2 (\hat{n} \cdot \vec{v}_2)^2 - \frac{15}{4} (\hat{n} \cdot \vec{S}_1)^2 \vec{v}_1 \cdot \vec{v}_2 (\hat{n} \cdot \vec{v}_2)^2 - \frac{1}{2} \vec{S}_1 \cdot \vec{S}_1 \vec{v}_1 \cdot \vec{v}_2 (\hat{n} \cdot \vec{v}_2)^2 + 2 \hat{n} \cdot \vec{v}_1 (\vec{S}_1 \cdot \vec{v}_2)^2 \hat{n} \cdot \vec{v}_2 + \right. \right. \\
 \left. \left. \frac{7}{2} \hat{n} \cdot \vec{S}_1 \vec{S}_1 \cdot \vec{v}_2 \vec{v}_1 \cdot \vec{v}_2 \hat{n} \cdot \vec{v}_2 - \frac{15}{2} (\hat{n} \cdot \vec{S}_1)^2 \hat{n} \cdot \vec{v}_1 \vec{v}_2 \cdot \vec{v}_2 \hat{n} \cdot \vec{v}_2 + \frac{5}{2} \hat{n} \cdot \vec{S}_1 \vec{S}_1 \cdot \vec{v}_1 \vec{v}_2 \cdot \vec{v}_2 \hat{n} \cdot \vec{v}_2 - \right. \right. \\
 \left. \left. \frac{1}{2} (\vec{S}_1 \cdot \vec{v}_2)^2 \vec{v}_1 \cdot \vec{v}_2 + 3 \hat{n} \cdot \vec{S}_1 \hat{n} \cdot \vec{v}_1 \vec{S}_1 \cdot \vec{v}_2 \vec{v}_2 \cdot \vec{v}_2 - \frac{3}{4} \vec{S}_1 \cdot \vec{v}_1 \vec{S}_1 \cdot \vec{v}_2 \vec{v}_2 \cdot \vec{v}_2 + \frac{5}{4} (\hat{n} \cdot \vec{S}_1)^2 \vec{v}_1 \cdot \vec{v}_2 \vec{v}_2 \cdot \vec{v}_2 \right) \right) m_2 C_{ES^2_1} \}
 \end{aligned}$$

{DiagS1CES2[2, 2, 60],

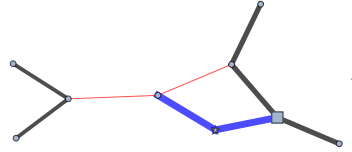

,

$$\begin{aligned}
 G^2 \left( \frac{1}{r} \left( 6 \hat{n} \cdot \vec{S}_1 \hat{n} \cdot \vec{S}_1 \hat{n} \cdot \vec{v}_1 + 2 \hat{n} \cdot \vec{S}_1 \hat{n} \cdot \vec{S}_1 \hat{n} \cdot \vec{v}_1 + 3 \vec{S}_1 \cdot \vec{S}_1 \hat{n} \cdot \vec{v}_1 + \vec{S}_1 \cdot \vec{S}_1 \hat{n} \cdot \vec{v}_1 - 4 \hat{n} \cdot \vec{S}_1 \hat{n} \cdot \vec{S}_1 \hat{n} \cdot \vec{v}_2 - \right. \right. \\
 \left. \left. \frac{4}{3} \hat{n} \cdot \vec{S}_1 \hat{n} \cdot \vec{S}_1 \hat{n} \cdot \vec{v}_2 - 4 \hat{n} \cdot \vec{v}_2 \vec{S}_1 \cdot \vec{S}_1 - \frac{3}{2} \hat{n} \cdot \vec{S}_1 \vec{S}_1 \cdot \vec{v}_1 + 2 \hat{n} \cdot \vec{S}_1 \vec{S}_1 \cdot \vec{v}_2 - \frac{3}{2} \hat{n} \cdot \vec{S}_1 \vec{S}_1 \cdot \vec{v}_1 + \right. \right. \\
 \left. \left. 2 \hat{n} \cdot \vec{S}_1 \vec{S}_1 \cdot \vec{v}_2 - \frac{1}{2} \hat{n} \cdot \vec{S}_1 \vec{S}_1 \cdot \vec{v}_1 + \frac{2}{3} \hat{n} \cdot \vec{S}_1 \vec{S}_1 \cdot \vec{v}_2 - \frac{4}{3} \hat{n} \cdot \vec{v}_2 \vec{S}_1 \cdot \vec{S}_1 - \frac{1}{2} \hat{n} \cdot \vec{S}_1 \vec{S}_1 \cdot \vec{v}_1 + \frac{2}{3} \hat{n} \cdot \vec{S}_1 \vec{S}_1 \cdot \vec{v}_2 \right) + \right. \\
 \left. \frac{1}{r^2} \left( 6 (\hat{n} \cdot \vec{v}_1)^2 (\hat{n} \cdot \vec{S}_1)^2 - 8 \hat{n} \cdot \vec{v}_1 \hat{n} \cdot \vec{v}_2 (\hat{n} \cdot \vec{S}_1)^2 - \frac{1}{2} \vec{v}_1 \cdot \vec{v}_1 (\hat{n} \cdot \vec{S}_1)^2 + 2 \vec{v}_1 \cdot \vec{v}_2 (\hat{n} \cdot \vec{S}_1)^2 + \right. \right. \\
 \left. \left. 6 \hat{n} \cdot \vec{a}_1 \hat{n} \cdot \vec{S}_1 \hat{n} \cdot \vec{v}_1 \hat{n} \cdot \vec{S}_1 - 8 \hat{n} \cdot \vec{a}_1 \hat{n} \cdot \vec{S}_1 \hat{n} \cdot \vec{v}_2 \hat{n} \cdot \vec{S}_1 - \hat{n} \cdot \vec{v}_1 \vec{S}_1 \cdot \vec{v}_1 \hat{n} \cdot \vec{S}_1 + 4 \hat{n} \cdot \vec{v}_1 \vec{S}_1 \cdot \vec{v}_2 \hat{n} \cdot \vec{S}_1 + \right. \right. \\
 \left. \left. 2 \hat{n} \cdot \vec{S}_1 \vec{a}_1 \cdot \vec{v}_2 \hat{n} \cdot \vec{S}_1 - \frac{3}{4} \hat{n} \cdot \vec{v}_1 \vec{S}_1 \cdot \vec{a}_1 \hat{n} \cdot \vec{S}_1 + \hat{n} \cdot \vec{v}_2 \vec{S}_1 \cdot \vec{a}_1 \hat{n} \cdot \vec{S}_1 + \frac{5}{4} \hat{n} \cdot \vec{a}_1 \vec{S}_1 \cdot \vec{v}_1 \hat{n} \cdot \vec{S}_1 + 2 \hat{n} \cdot \vec{a}_1 \vec{S}_1 \cdot \vec{v}_2 \hat{n} \cdot \vec{S}_1 - \right. \right. \\
 \left. \left. 4 \hat{n} \cdot \vec{S}_1 \vec{v}_1 \cdot \vec{a}_1 \hat{n} \cdot \vec{S}_1 + 6 \hat{n} \cdot \vec{S}_1 \hat{n} \cdot \vec{S}_1 (\hat{n} \cdot \vec{v}_1)^2 - \left( \vec{S}_1 \cdot \vec{v}_1 \right)^2 + \hat{n} \cdot \vec{a}_1 (\hat{n} \cdot \vec{S}_1)^2 \hat{n} \cdot \vec{v}_1 - \frac{4}{3} \hat{n} \cdot \vec{a}_1 (\hat{n} \cdot \vec{S}_1)^2 \hat{n} \cdot \vec{v}_2 - \right. \right. \\
 \left. \left. \frac{1}{3} \hat{n} \cdot \vec{a}_1 (\hat{n} \cdot \vec{S}_1)^2 \hat{n} \cdot \vec{v}_2 - \frac{1}{3} \hat{n} \cdot \vec{a}_1 (\hat{n} \cdot \vec{S}_1)^2 \hat{n} \cdot \vec{v}_2 \right) \right) m_2 C_{ES^2_1} \}
 \end{aligned}$$



{DiagS1CES2[2, 2, 61],

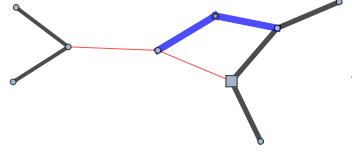

$$\begin{aligned}
 & G^2 \left( \frac{1}{\rho^2} \left( -20 \hat{n} \cdot \vec{S}_1 \hat{n} \cdot \vec{a}_1 \hat{n} \cdot \vec{S}_1 \hat{n} \cdot \vec{v}_1 + \frac{7}{2} \hat{n} \cdot \vec{S}_1 \vec{S}_1 \cdot \vec{a}_1 \hat{n} \cdot \vec{v}_1 + 2 \hat{n} \cdot \vec{a}_1 \vec{S}_1 \cdot \vec{S}_1 \hat{n} \cdot \vec{v}_1 + \frac{7}{2} \hat{n} \cdot \vec{S}_1 \vec{S}_1 \cdot \vec{a}_1 \hat{n} \cdot \vec{v}_1 + \frac{7}{2} \hat{n} \cdot \vec{a}_1 \hat{n} \cdot \vec{S}_1 \right. \right. \\
 & \quad \left. \left. \vec{S}_1 \cdot \vec{v}_1 - \vec{S}_1 \cdot \vec{v}_1 \vec{S}_1 \cdot \vec{a}_1 + \frac{7}{2} \hat{n} \cdot \vec{S}_1 \hat{n} \cdot \vec{a}_1 \vec{S}_1 \cdot \vec{v}_1 - \vec{S}_1 \cdot \vec{a}_1 \vec{S}_1 \cdot \vec{v}_1 + 5 \hat{n} \cdot \vec{S}_1 \hat{n} \cdot \vec{S}_1 \vec{v}_1 \cdot \vec{a}_1 - \vec{S}_1 \cdot \vec{S}_1 \vec{v}_1 \cdot \vec{a}_1 \right) + \frac{1}{\rho^3} \right. \\
 & \quad \left( -10 \hat{n} \cdot \vec{S}_1 \hat{n} \cdot \vec{S}_1 (\hat{n} \cdot \vec{v}_1)^3 + \frac{8}{3} \vec{S}_1 \cdot \vec{S}_1 (\hat{n} \cdot \vec{v}_1)^3 + 70 \hat{n} \cdot \vec{a}_1 (\hat{n} \cdot \vec{S}_1)^2 (\hat{n} \cdot \vec{v}_1)^2 + \hat{n} \cdot \vec{S}_1 \vec{S}_1 \cdot \vec{v}_1 (\hat{n} \cdot \vec{v}_1)^2 - \right. \\
 & \quad \frac{55}{3} \hat{n} \cdot \vec{S}_1 \vec{S}_1 \cdot \vec{a}_1 (\hat{n} \cdot \vec{v}_1)^2 - \frac{20}{3} \hat{n} \cdot \vec{a}_1 \vec{S}_1 \cdot \vec{S}_1 (\hat{n} \cdot \vec{v}_1)^2 + \hat{n} \cdot \vec{S}_1 \vec{S}_1 \cdot \vec{v}_1 (\hat{n} \cdot \vec{v}_1)^2 - \\
 & \quad 60 \hat{n} \cdot \vec{a}_1 (\hat{n} \cdot \vec{S}_1)^2 \hat{n} \cdot \vec{v}_2 \hat{n} \cdot \vec{v}_1 + 10 (\hat{n} \cdot \vec{S}_1)^2 \vec{a}_1 \cdot \vec{v}_2 \hat{n} \cdot \vec{v}_1 + 14 \hat{n} \cdot \vec{S}_1 \hat{n} \cdot \vec{v}_2 \vec{S}_1 \cdot \vec{a}_1 \hat{n} \cdot \vec{v}_1 + \\
 & \quad 4 \hat{n} \cdot \vec{a}_1 \hat{n} \cdot \vec{v}_2 \vec{S}_1 \cdot \vec{S}_1 \hat{n} \cdot \vec{v}_1 - \vec{a}_1 \cdot \vec{v}_2 \vec{S}_1 \cdot \vec{S}_1 \hat{n} \cdot \vec{v}_1 - \frac{95}{3} \hat{n} \cdot \vec{a}_1 \hat{n} \cdot \vec{S}_1 \vec{S}_1 \cdot \vec{v}_1 \hat{n} \cdot \vec{v}_1 + \frac{1}{\vec{S}_1 \cdot \vec{v}_1 \vec{S}_1 \cdot \vec{v}_1} \hat{n} \cdot \vec{v}_1 + \\
 & \quad \frac{17}{3} \vec{S}_1 \cdot \vec{a}_1 \vec{S}_1 \cdot \vec{v}_1 \hat{n} \cdot \vec{v}_1 + 20 \hat{n} \cdot \vec{a}_1 \hat{n} \cdot \vec{S}_1 \vec{S}_1 \cdot \vec{v}_2 \hat{n} \cdot \vec{v}_1 - \frac{7}{2} \vec{S}_1 \cdot \vec{a}_1 \vec{S}_1 \cdot \vec{v}_2 \hat{n} \cdot \vec{v}_1 - \frac{125}{6} (\hat{n} \cdot \vec{S}_1)^2 \vec{v}_1 \cdot \vec{a}_1 \hat{n} \cdot \vec{v}_1 + \\
 & \quad \frac{17}{6} \vec{S}_1 \cdot \vec{S}_1 \vec{v}_1 \cdot \vec{a}_1 \hat{n} \cdot \vec{v}_1 - \vec{S}_1 \cdot \vec{S}_1 \vec{v}_1 \cdot \vec{v}_1 \hat{n} \cdot \vec{v}_1 + \frac{7}{3} \hat{n} \cdot \vec{a}_1 (\vec{S}_1 \cdot \vec{v}_1)^2 + 14 \hat{n} \cdot \vec{a}_1 \hat{n} \cdot \vec{S}_1 \hat{n} \cdot \vec{v}_2 \vec{S}_1 \cdot \vec{v}_1 - \\
 & \quad \frac{7}{2} \hat{n} \cdot \vec{S}_1 \vec{a}_1 \cdot \vec{v}_2 \vec{S}_1 \cdot \vec{v}_1 - 2 \hat{n} \cdot \vec{v}_2 \vec{S}_1 \cdot \vec{a}_1 \vec{S}_1 \cdot \vec{v}_1 - \frac{7}{2} \hat{n} \cdot \vec{a}_1 \vec{S}_1 \cdot \vec{v}_1 \vec{S}_1 \cdot \vec{v}_2 + 10 (\hat{n} \cdot \vec{S}_1)^2 \hat{n} \cdot \vec{v}_2 \vec{v}_1 \cdot \vec{a}_1 - \\
 & \quad \hat{n} \cdot \vec{v}_2 \vec{S}_1 \cdot \vec{S}_1 \vec{v}_1 \cdot \vec{a}_1 + \frac{20}{3} \hat{n} \cdot \vec{S}_1 \vec{S}_1 \cdot \vec{v}_1 \vec{v}_1 \cdot \vec{a}_1 - 5 \hat{n} \cdot \vec{S}_1 \vec{S}_1 \cdot \vec{v}_2 \vec{v}_1 \cdot \vec{a}_1 - \frac{55}{6} \hat{n} \cdot \vec{a}_1 (\hat{n} \cdot \vec{S}_1)^2 \vec{v}_1 \cdot \vec{v}_1 + \\
 & \quad \hat{n} \cdot \vec{S}_1 \vec{S}_1 \cdot \vec{v}_1 \vec{v}_1 \cdot \vec{v}_1 + \frac{10}{3} \hat{n} \cdot \vec{S}_1 \vec{S}_1 \cdot \vec{a}_1 \vec{v}_1 \cdot \vec{v}_1 + \frac{7}{6} \hat{n} \cdot \vec{a}_1 \vec{S}_1 \cdot \vec{S}_1 \vec{v}_1 \cdot \vec{v}_1 + \hat{n} \cdot \vec{S}_1 \vec{S}_1 \cdot \vec{v}_1 \vec{v}_1 \cdot \vec{v}_1 + \\
 & \quad \left. 10 \hat{n} \cdot \vec{a}_1 (\hat{n} \cdot \vec{S}_1)^2 \vec{v}_1 \cdot \vec{v}_2 - \frac{7}{2} \hat{n} \cdot \vec{S}_1 \vec{S}_1 \cdot \vec{a}_1 \vec{v}_1 \cdot \vec{v}_2 - \hat{n} \cdot \vec{a}_1 \vec{S}_1 \cdot \vec{S}_1 \vec{v}_1 \cdot \vec{v}_2 \right) + \frac{1}{\rho^4} \\
 & \quad \left( 35 (\hat{n} \cdot \vec{S}_1)^2 (\hat{n} \cdot \vec{v}_1)^4 - \frac{25}{4} \vec{S}_1 \cdot \vec{S}_1 (\hat{n} \cdot \vec{v}_1)^4 - 40 (\hat{n} \cdot \vec{S}_1)^2 \hat{n} \cdot \vec{v}_2 (\hat{n} \cdot \vec{v}_1)^3 + 8 \hat{n} \cdot \vec{v}_2 \vec{S}_1 \cdot \vec{S}_1 (\hat{n} \cdot \vec{v}_1)^3 - \right. \\
 & \quad \frac{65}{4} \hat{n} \cdot \vec{S}_1 \vec{S}_1 \cdot \vec{v}_1 (\hat{n} \cdot \vec{v}_1)^3 + 10 \hat{n} \cdot \vec{S}_1 \vec{S}_1 \cdot \vec{v}_2 (\hat{n} \cdot \vec{v}_1)^3 + \frac{1}{4} (\vec{S}_1 \cdot \vec{v}_1)^2 (\hat{n} \cdot \vec{v}_1)^2 + \\
 & \quad 6 \hat{n} \cdot \vec{S}_1 \hat{n} \cdot \vec{v}_2 \vec{S}_1 \cdot \vec{v}_1 (\hat{n} \cdot \vec{v}_1)^2 - \vec{S}_1 \cdot \vec{v}_1 \vec{S}_1 \cdot \vec{v}_2 (\hat{n} \cdot \vec{v}_1)^2 - \frac{15}{8} (\hat{n} \cdot \vec{S}_1)^2 \vec{v}_1 \cdot \vec{v}_1 (\hat{n} \cdot \vec{v}_1)^2 + \\
 & \quad \frac{21}{8} \vec{S}_1 \cdot \vec{S}_1 \vec{v}_1 \cdot \vec{v}_1 (\hat{n} \cdot \vec{v}_1)^2 + 15 (\hat{n} \cdot \vec{S}_1)^2 \vec{v}_1 \cdot \vec{v}_2 (\hat{n} \cdot \vec{v}_1)^2 - 4 \vec{S}_1 \cdot \vec{S}_1 \vec{v}_1 \cdot \vec{v}_2 (\hat{n} \cdot \vec{v}_1)^2 + \\
 & \quad 2 \hat{n} \cdot \vec{v}_2 (\vec{S}_1 \cdot \vec{v}_1)^2 \hat{n} \cdot \vec{v}_1 - 2 \hat{n} \cdot \vec{v}_2 \vec{S}_1 \cdot \vec{S}_1 \vec{v}_1 \cdot \vec{v}_1 \hat{n} \cdot \vec{v}_1 - \frac{25}{4} \hat{n} \cdot \vec{S}_1 \vec{S}_1 \cdot \vec{v}_1 \vec{v}_1 \cdot \vec{v}_1 \hat{n} \cdot \vec{v}_1 - \\
 & \quad 2 \hat{n} \cdot \vec{S}_1 \vec{S}_1 \cdot \vec{v}_1 \vec{v}_1 \cdot \vec{v}_2 \hat{n} \cdot \vec{v}_1 - \frac{15}{8} (\hat{n} \cdot \vec{S}_1)^2 (\vec{v}_1 \cdot \vec{v}_1)^2 + \frac{1}{8} \vec{S}_1 \cdot \vec{S}_1 (\vec{v}_1 \cdot \vec{v}_1)^2 + \frac{3}{2} (\vec{S}_1 \cdot \vec{v}_1)^2 \vec{v}_1 \cdot \vec{v}_1 + \\
 & \quad \left. 4 \hat{n} \cdot \vec{S}_1 \hat{n} \cdot \vec{v}_2 \vec{S}_1 \cdot \vec{v}_1 \vec{v}_1 \cdot \vec{v}_1 - \vec{S}_1 \cdot \vec{v}_1 \vec{S}_1 \cdot \vec{v}_2 \vec{v}_1 \cdot \vec{v}_1 - \frac{1}{2} (\vec{S}_1 \cdot \vec{v}_1)^2 \vec{v}_1 \cdot \vec{v}_2 + \frac{1}{2} \vec{S}_1 \cdot \vec{S}_1 \vec{v}_1 \cdot \vec{v}_1 \vec{v}_1 \cdot \vec{v}_2 \right) \Big) m_2 C_{ES^2_1} \Big\}
 \end{aligned}$$

{DiagS1CES2[2, 2, 62],

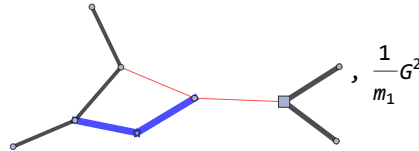

$$\begin{aligned}
 & \left( \frac{1}{\rho^2} \left( -\frac{32}{3} \hat{n} \cdot \vec{S}_1 \hat{n} \cdot \vec{a}_2 \hat{n} \cdot \vec{S}_1 \hat{n} \cdot \vec{v}_2 + \frac{8}{3} \hat{n} \cdot \vec{S}_1 \vec{S}_1 \cdot \vec{a}_2 \hat{n} \cdot \vec{v}_2 - \frac{16}{3} \hat{n} \cdot \vec{a}_2 \vec{S}_1 \cdot \vec{S}_1 \hat{n} \cdot \vec{v}_2 + \frac{8}{3} \hat{n} \cdot \vec{S}_1 \vec{S}_1 \cdot \vec{a}_2 \hat{n} \cdot \vec{v}_2 + \frac{8}{3} \hat{n} \cdot \vec{a}_2 \hat{n} \cdot \vec{S}_1 \right. \right. \\
 & \quad \left. \left. \vec{S}_1 \cdot \vec{v}_2 - \frac{4}{3} \vec{S}_1 \cdot \vec{v}_2 \vec{S}_1 \cdot \vec{a}_2 + \frac{8}{3} \hat{n} \cdot \vec{S}_1 \hat{n} \cdot \vec{a}_2 \vec{S}_1 \cdot \vec{v}_2 - \frac{4}{3} \vec{S}_1 \cdot \vec{a}_2 \vec{S}_1 \cdot \vec{v}_2 + \frac{8}{3} \hat{n} \cdot \vec{S}_1 \hat{n} \cdot \vec{S}_1 \vec{v}_2 \cdot \vec{a}_2 + \frac{8}{3} \vec{S}_1 \cdot \vec{S}_1 \vec{v}_2 \cdot \vec{a}_2 \right) + \frac{1}{\rho^3} \right.
 \end{aligned}$$



$$\begin{aligned}
& \left( 16 \hat{n} \cdot \vec{S}_1 \hat{n} \cdot \vec{S}_1 (\hat{n} \cdot \vec{v}_2)^3 + \frac{16}{3} \vec{S}_1 \cdot \vec{S}_1 (\hat{n} \cdot \vec{v}_2)^3 - 48 \hat{n} \cdot \vec{a}_2 (\hat{n} \cdot \vec{S}_1)^2 (\hat{n} \cdot \vec{v}_2)^2 - 8 \hat{n} \cdot \vec{S}_1 \vec{S}_1 \cdot \vec{v}_2 (\hat{n} \cdot \vec{v}_2)^2 + \right. \\
& 16 \hat{n} \cdot \vec{S}_1 \vec{S}_1 \cdot \vec{a}_2 (\hat{n} \cdot \vec{v}_2)^2 - 16 \hat{n} \cdot \vec{a}_2 \vec{S}_1 \cdot \vec{S}_1 (\hat{n} \cdot \vec{v}_2)^2 - 8 \hat{n} \cdot \vec{S}_1 \vec{S}_1 \cdot \vec{v}_2 (\hat{n} \cdot \vec{v}_2)^2 + 32 \hat{n} \cdot \vec{a}_2 (\hat{n} \cdot \vec{S}_1)^2 \hat{n} \cdot \vec{v}_1 \hat{n} \cdot \vec{v}_2 - \\
& \frac{32}{3} \hat{n} \cdot \vec{S}_1 \hat{n} \cdot \vec{v}_1 \vec{S}_1 \cdot \vec{a}_2 \hat{n} \cdot \vec{v}_2 + \frac{32}{3} \hat{n} \cdot \vec{a}_2 \hat{n} \cdot \vec{v}_1 \vec{S}_1 \cdot \vec{S}_1 \hat{n} \cdot \vec{v}_2 - \frac{32}{3} \hat{n} \cdot \vec{a}_2 \hat{n} \cdot \vec{S}_1 \vec{S}_1 \cdot \vec{v}_1 \hat{n} \cdot \vec{v}_2 + \\
& \frac{8}{3} \vec{S}_1 \cdot \vec{a}_2 \vec{S}_1 \cdot \vec{v}_1 \hat{n} \cdot \vec{v}_2 + 32 \hat{n} \cdot \vec{a}_2 \hat{n} \cdot \vec{S}_1 \vec{S}_1 \cdot \vec{v}_2 \hat{n} \cdot \vec{v}_2 + 4 \vec{S}_1 \cdot \vec{v}_2 \vec{S}_1 \cdot \vec{v}_2 \hat{n} \cdot \vec{v}_2 - 8 \vec{S}_1 \cdot \vec{a}_2 \vec{S}_1 \cdot \vec{v}_2 \hat{n} \cdot \vec{v}_2 - \\
& \frac{16}{3} (\hat{n} \cdot \vec{S}_1)^2 \vec{v}_1 \cdot \vec{a}_2 \hat{n} \cdot \vec{v}_2 - \frac{8}{3} \vec{S}_1 \cdot \vec{S}_1 \vec{v}_1 \cdot \vec{a}_2 \hat{n} \cdot \vec{v}_2 + 12 (\hat{n} \cdot \vec{S}_1)^2 \vec{v}_2 \cdot \vec{a}_2 \hat{n} \cdot \vec{v}_2 + 8 \vec{S}_1 \cdot \vec{S}_1 \vec{v}_2 \cdot \vec{a}_2 \hat{n} \cdot \vec{v}_2 - \\
& 4 \vec{S}_1 \cdot \vec{S}_1 \vec{v}_2 \cdot \vec{v}_2 \hat{n} \cdot \vec{v}_2 - 4 \hat{n} \cdot \vec{a}_2 (\vec{S}_1 \cdot \vec{v}_2)^2 - \frac{32}{3} \hat{n} \cdot \vec{a}_2 \hat{n} \cdot \vec{S}_1 \hat{n} \cdot \vec{v}_1 \vec{S}_1 \cdot \vec{v}_2 + \frac{8}{3} \hat{n} \cdot \vec{v}_1 \vec{S}_1 \cdot \vec{a}_2 \vec{S}_1 \cdot \vec{v}_2 + \\
& \frac{8}{3} \hat{n} \cdot \vec{a}_2 \vec{S}_1 \cdot \vec{v}_1 \vec{S}_1 \cdot \vec{v}_2 + \frac{8}{3} \hat{n} \cdot \vec{S}_1 \vec{S}_1 \cdot \vec{v}_2 \vec{v}_1 \cdot \vec{a}_2 - \frac{16}{3} \hat{n} \cdot \vec{a}_2 (\hat{n} \cdot \vec{S}_1)^2 \vec{v}_1 \cdot \vec{v}_2 + \frac{8}{3} \hat{n} \cdot \vec{S}_1 \vec{S}_1 \cdot \vec{a}_2 \vec{v}_1 \cdot \vec{v}_2 - \\
& \frac{8}{3} \hat{n} \cdot \vec{a}_2 \vec{S}_1 \cdot \vec{S}_1 \vec{v}_1 \cdot \vec{v}_2 - \frac{16}{3} (\hat{n} \cdot \vec{S}_1)^2 \hat{n} \cdot \vec{v}_1 \vec{v}_2 \cdot \vec{a}_2 - \frac{8}{3} \hat{n} \cdot \vec{v}_1 \vec{S}_1 \cdot \vec{S}_1 \vec{v}_2 \cdot \vec{a}_2 + \frac{8}{3} \hat{n} \cdot \vec{S}_1 \vec{S}_1 \cdot \vec{v}_1 \vec{v}_2 \cdot \vec{a}_2 - \\
& 6 \hat{n} \cdot \vec{S}_1 \vec{S}_1 \cdot \vec{v}_2 \vec{v}_2 \cdot \vec{a}_2 + 4 \hat{n} \cdot \vec{a}_2 (\hat{n} \cdot \vec{S}_1)^2 \vec{v}_2 \cdot \vec{v}_2 - 2 \hat{n} \cdot \vec{S}_1 \vec{S}_1 \cdot \vec{a}_2 \vec{v}_2 \cdot \vec{v}_2 + 4 \hat{n} \cdot \vec{a}_2 \vec{S}_1 \cdot \vec{S}_1 \vec{v}_2 \cdot \vec{v}_2 \Big) + \frac{1}{r^4} \\
& \left( 48 (\hat{n} \cdot \vec{S}_1)^2 (\hat{n} \cdot \vec{v}_2)^4 + 12 \vec{S}_1 \cdot \vec{S}_1 (\hat{n} \cdot \vec{v}_2)^4 - 64 (\hat{n} \cdot \vec{S}_1)^2 \hat{n} \cdot \vec{v}_1 (\hat{n} \cdot \vec{v}_2)^3 - 16 \hat{n} \cdot \vec{v}_1 \vec{S}_1 \cdot \vec{S}_1 (\hat{n} \cdot \vec{v}_2)^3 + \right. \\
& 16 \hat{n} \cdot \vec{S}_1 \vec{S}_1 \cdot \vec{v}_1 (\hat{n} \cdot \vec{v}_2)^3 - 48 \hat{n} \cdot \vec{S}_1 \vec{S}_1 \cdot \vec{v}_2 (\hat{n} \cdot \vec{v}_2)^3 + 12 (\vec{S}_1 \cdot \vec{v}_2)^2 (\hat{n} \cdot \vec{v}_2)^2 + \\
& 48 \hat{n} \cdot \vec{S}_1 \hat{n} \cdot \vec{v}_1 \vec{S}_1 \cdot \vec{v}_2 (\hat{n} \cdot \vec{v}_2)^2 - 8 \vec{S}_1 \cdot \vec{v}_1 \vec{S}_1 \cdot \vec{v}_2 (\hat{n} \cdot \vec{v}_2)^2 + 24 (\hat{n} \cdot \vec{S}_1)^2 \vec{v}_1 \cdot \vec{v}_2 (\hat{n} \cdot \vec{v}_2)^2 + \\
& 8 \vec{S}_1 \cdot \vec{S}_1 \vec{v}_1 \cdot \vec{v}_2 (\hat{n} \cdot \vec{v}_2)^2 - 6 (\hat{n} \cdot \vec{S}_1)^2 \vec{v}_2 \cdot \vec{v}_2 (\hat{n} \cdot \vec{v}_2)^2 - 12 \vec{S}_1 \cdot \vec{S}_1 \vec{v}_2 \cdot \vec{v}_2 (\hat{n} \cdot \vec{v}_2)^2 - 8 \hat{n} \cdot \vec{v}_1 (\vec{S}_1 \cdot \vec{v}_2)^2 \hat{n} \cdot \vec{v}_2 - \\
& 16 \hat{n} \cdot \vec{S}_1 \vec{S}_1 \cdot \vec{v}_2 \vec{v}_1 \cdot \vec{v}_2 \hat{n} \cdot \vec{v}_2 + 8 \hat{n} \cdot \vec{v}_1 \vec{S}_1 \cdot \vec{S}_1 \vec{v}_2 \cdot \vec{v}_2 \hat{n} \cdot \vec{v}_2 + 4 \hat{n} \cdot \vec{S}_1 \vec{S}_1 \cdot \vec{v}_2 \vec{v}_2 \cdot \vec{v}_2 \hat{n} \cdot \vec{v}_2 - 2 (\hat{n} \cdot \vec{S}_1)^2 (\vec{v}_2 \cdot \vec{v}_2)^2 + \\
& \left. \frac{3}{2} \vec{S}_1 \cdot \vec{S}_1 (\vec{v}_2 \cdot \vec{v}_2)^2 + 2 (\vec{S}_1 \cdot \vec{v}_2)^2 \vec{v}_1 \cdot \vec{v}_2 - \frac{1}{2} (\vec{S}_1 \cdot \vec{v}_2)^2 \vec{v}_2 \cdot \vec{v}_2 - 2 \vec{S}_1 \cdot \vec{S}_1 \vec{v}_1 \cdot \vec{v}_2 \vec{v}_2 \cdot \vec{v}_2 \right) \Big) m_{\text{ES}^2}^2 \}
\end{aligned}$$

{DiagS1CES2[2, 2, 63],

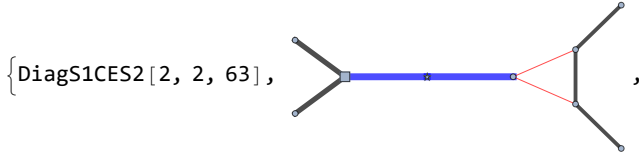

,

$$\begin{aligned}
& \frac{1}{m_1} G^2 \left( \frac{1}{r} \left( -\frac{1}{2} \hat{n} \cdot \vec{S}_1 \hat{n} \cdot \vec{S}_1 \hat{n} \cdot \vec{v}_2 - \frac{1}{6} \hat{n} \cdot \vec{S}_1^3 \hat{n} \cdot \vec{S}_1 \hat{n} \cdot \vec{v}_2 - 2 \vec{S}_1 \cdot \vec{S}_1 \hat{n} \cdot \vec{v}_2 - \right. \right. \\
& \left. \frac{2}{3} \vec{S}_1 \cdot \vec{S}_1^3 \hat{n} \cdot \vec{v}_2 + \frac{1}{4} \hat{n} \cdot \vec{S}_1 \vec{S}_1 \cdot \vec{v}_2 + \frac{1}{4} \hat{n} \cdot \vec{S}_1 \vec{S}_1^2 \cdot \vec{v}_2 + \frac{1}{12} \hat{n} \cdot \vec{S}_1 \vec{S}_1^3 \cdot \vec{v}_2 + \frac{1}{12} \hat{n} \cdot \vec{S}_1^3 \vec{S}_1 \cdot \vec{v}_2 \right) + \frac{1}{r^2} \\
& \left( 2 \hat{n} \cdot \vec{v}_1 \hat{n} \cdot \vec{v}_2 (\hat{n} \cdot \vec{S}_1)^2 - \frac{1}{2} \vec{v}_1 \cdot \vec{v}_2 (\hat{n} \cdot \vec{S}_1)^2 + 2 \hat{n} \cdot \vec{a}_1 \hat{n} \cdot \vec{S}_1 \hat{n} \cdot \vec{v}_2 \hat{n} \cdot \vec{S}_1 - 2 \hat{n} \cdot \vec{v}_2 \vec{S}_1 \cdot \vec{v}_1 \hat{n} \cdot \vec{S}_1 - \right. \\
& \hat{n} \cdot \vec{v}_1 \vec{S}_1 \cdot \vec{v}_2 \hat{n} \cdot \vec{S}_1 - \frac{1}{2} \hat{n} \cdot \vec{S}_1 \vec{a}_1 \cdot \vec{v}_2 \hat{n} \cdot \vec{S}_1 - \frac{3}{2} \hat{n} \cdot \vec{v}_2 \vec{S}_1 \cdot \vec{a}_1 \hat{n} \cdot \vec{S}_1 - \frac{1}{2} \hat{n} \cdot \vec{a}_1 \vec{S}_1 \cdot \vec{v}_2 \hat{n} \cdot \vec{S}_1 + \frac{1}{3} \hat{n} \cdot \vec{a}_1 (\hat{n} \cdot \vec{S}_1)^2 \hat{n} \cdot \vec{v}_2 + \\
& 2 \hat{n} \cdot \vec{S}_1 \hat{n} \cdot \vec{S}_1 \hat{n} \cdot \vec{v}_1 \hat{n} \cdot \vec{v}_2 - \frac{1}{12} (\hat{n} \cdot \vec{S}_1)^2 \vec{a}_1 \cdot \vec{v}_2 + 3 \hat{n} \cdot \vec{v}_1 \hat{n} \cdot \vec{v}_2 \vec{S}_1 \cdot \vec{S}_1 - \frac{3}{2} \hat{n} \cdot \vec{S}_1 \hat{n} \cdot \vec{v}_2 \vec{S}_1 \cdot \vec{a}_1 - \\
& \frac{1}{2} \hat{n} \cdot \vec{a}_1 \hat{n} \cdot \vec{S}_1 \vec{S}_1 \cdot \vec{v}_2 + \vec{S}_1 \cdot \vec{v}_1 \vec{S}_1 \cdot \vec{v}_2 - \hat{n} \cdot \vec{S}_1 \hat{n} \cdot \vec{v}_2 \vec{S}_1 \cdot \vec{v}_1 - \frac{1}{2} \hat{n} \cdot \vec{S}_1 \hat{n} \cdot \vec{v}_1 \vec{S}_1 \cdot \vec{v}_2 - \frac{2}{3} \hat{n} \cdot \vec{S}_1 \hat{n} \cdot \vec{v}_2 \vec{S}_1 \cdot \vec{a}_1 + \\
& 2 \hat{n} \cdot \vec{a}_1 \hat{n} \cdot \vec{v}_2 \vec{S}_1 \cdot \vec{S}_1 - \vec{a}_1 \cdot \vec{v}_2 \vec{S}_1 \cdot \vec{S}_1 + 3 \hat{n} \cdot \vec{v}_1 \hat{n} \cdot \vec{v}_2 \vec{S}_1 \cdot \vec{S}_1 + \frac{3}{4} \vec{S}_1 \cdot \vec{v}_2 \vec{S}_1 \cdot \vec{a}_1 + \frac{1}{6} \hat{n} \cdot \vec{a}_1 \hat{n} \cdot \vec{v}_2 \vec{S}_1 \cdot \vec{S}_1 - \\
& \frac{1}{12} \vec{a}_1 \cdot \vec{v}_2 \vec{S}_1 \cdot \vec{S}_1 - \hat{n} \cdot \vec{S}_1 \hat{n} \cdot \vec{v}_2 \vec{S}_1 \cdot \vec{v}_1 + \frac{1}{2} \vec{S}_1 \cdot \vec{v}_2 \vec{S}_1 \cdot \vec{v}_1 - \frac{1}{6} \hat{n} \cdot \vec{a}_1 \hat{n} \cdot \vec{S}_1 \vec{S}_1 \cdot \vec{v}_2 - \frac{1}{2} \hat{n} \cdot \vec{S}_1 \hat{n} \cdot \vec{v}_1 \vec{S}_1 \cdot \vec{v}_2 + \\
& \left. \frac{3}{4} \vec{S}_1 \cdot \vec{a}_1 \vec{S}_1 \cdot \vec{v}_2 + \frac{1}{2} \vec{S}_1 \cdot \vec{v}_1 \vec{S}_1 \cdot \vec{v}_2 + \frac{1}{3} \vec{S}_1 \cdot \vec{a}_1 \vec{S}_1 \cdot \vec{v}_2 - \frac{1}{2} \hat{n} \cdot \vec{S}_1 \hat{n} \cdot \vec{S}_1 \vec{v}_1 \cdot \vec{v}_2 - \frac{3}{2} \vec{S}_1 \cdot \vec{S}_1 \vec{v}_1 \cdot \vec{v}_2 - \frac{3}{2} \vec{S}_1 \cdot \vec{S}_1 \vec{v}_1 \cdot \vec{v}_2 \right) +
\end{aligned}$$

$r$

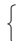

©

{DiagS1CES2[2, 2, 65],

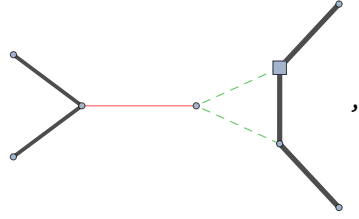

$$G^2 m_2 C_{ES^2 1} \left( \frac{1}{r^3} \left( -3 \hat{n} \cdot \vec{a}_1 \left( \vec{S}_1 \cdot \vec{v}_1 \right)^2 + \vec{S}_1 \cdot \vec{a}_1 \hat{n} \cdot \vec{v}_1 \vec{S}_1 \cdot \vec{v}_1 + 3 \vec{v}_1 \cdot \vec{a}_1 \hat{n} \cdot \vec{S}_1 \vec{S}_1 \cdot \vec{v}_1 - 3 \vec{v}_1 \cdot \vec{v}_1 \vec{S}_1 \cdot \vec{a}_1 \hat{n} \cdot \vec{S}_1 + \right. \right. \\ \left. \left. 6 \vec{S}_1 \cdot \vec{S}_1 \vec{v}_1 \cdot \vec{v}_1 \hat{n} \cdot \vec{a}_1 - 2 \hat{n} \cdot \vec{v}_1 \vec{S}_1 \cdot \vec{v}_1 \vec{S}_1 \cdot \vec{v}_1 + 3 \vec{v}_1 \cdot \vec{v}_1 \hat{n} \cdot \vec{S}_1 \vec{S}_1 \cdot \vec{v}_1 + 9 \vec{v}_2 \cdot \vec{v}_2 \hat{n} \cdot \vec{S}_1 \vec{S}_1 \cdot \vec{v}_1 + \right. \right. \\ \left. \left. 3 \vec{v}_1 \cdot \vec{v}_1 \hat{n} \cdot \vec{S}_1 \vec{S}_1 \cdot \vec{v}_1 + 4 \vec{S}_1 \cdot \vec{S}_1 \vec{v}_1 \cdot \vec{v}_1 \hat{n} \cdot \vec{v}_1 + 9 \vec{v}_2 \cdot \vec{v}_2 \hat{n} \cdot \vec{S}_1 \vec{S}_1 \cdot \vec{v}_1 - 6 \vec{S}_1 \cdot \vec{S}_1 \vec{v}_2 \cdot \vec{v}_2 \hat{n} \cdot \vec{v}_1 \right) + \right. \\ \left. \frac{1}{r^4} \left( -12 \left( \vec{v}_1 \cdot \vec{v}_1 \right)^2 \left( \hat{n} \cdot \vec{S}_1 \right)^2 - 18 \vec{v}_1 \cdot \vec{v}_1 \vec{v}_2 \cdot \vec{v}_2 \left( \hat{n} \cdot \vec{S}_1 \right)^2 + 12 \vec{v}_1 \cdot \vec{v}_1 \hat{n} \cdot \vec{S}_1 \hat{n} \cdot \vec{v}_1 \vec{S}_1 \cdot \vec{v}_1 - \right. \right. \\ \left. \left. 12 \vec{S}_1 \cdot \vec{S}_1 \vec{v}_1 \cdot \vec{v}_1 \left( \hat{n} \cdot \vec{v}_1 \right)^2 + 8 \vec{S}_1 \cdot \vec{S}_1 \left( \vec{v}_1 \cdot \vec{v}_1 \right)^2 - 4 \vec{v}_1 \cdot \vec{v}_1 \left( \vec{S}_1 \cdot \vec{v}_1 \right)^2 + 6 \vec{S}_1 \cdot \vec{S}_1 \vec{v}_1 \cdot \vec{v}_1 \vec{v}_2 \cdot \vec{v}_2 \right) \right) \Bigg\}$$

{DiagS1CES2[2, 2, 66],

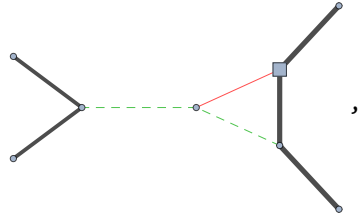

$$G^2 m_2 C_{ES^2 1} \left( \frac{1}{r^3} \left( -4 \vec{S}_1 \cdot \vec{a}_1 \hat{n} \cdot \vec{v}_2 \vec{S}_1 \cdot \vec{v}_1 + 4 \vec{S}_1 \cdot \vec{a}_1 \hat{n} \cdot \vec{v}_1 \vec{S}_1 \cdot \vec{v}_2 - \right. \right. \\ \left. \left. 8 \vec{v}_1 \cdot \vec{v}_2 \vec{S}_1 \cdot \vec{a}_1 \hat{n} \cdot \vec{S}_1 - 8 \hat{n} \cdot \vec{v}_2 \vec{S}_1 \cdot \vec{v}_1 \vec{S}_1 \cdot \vec{v}_1 + 4 \hat{n} \cdot \vec{v}_1 \vec{S}_1 \cdot \vec{v}_2 \vec{S}_1 \cdot \vec{v}_1 - 8 \vec{v}_1 \cdot \vec{v}_2 \hat{n} \cdot \vec{S}_1 \vec{S}_1 \cdot \vec{v}_1 + \right. \right. \\ \left. \left. 4 \hat{n} \cdot \vec{v}_1 \vec{S}_1 \cdot \vec{v}_1 \vec{S}_1 \cdot \vec{v}_2 + 8 \vec{S}_1 \cdot \vec{S}_1 \vec{v}_1 \cdot \vec{v}_1 \hat{n} \cdot \vec{v}_2 - 8 \vec{v}_1 \cdot \vec{v}_2 \hat{n} \cdot \vec{S}_1 \vec{S}_1 \cdot \vec{v}_1 + 8 \vec{S}_1 \cdot \vec{S}_1 \vec{v}_1 \cdot \vec{v}_2 \hat{n} \cdot \vec{v}_1 \right) + \right. \\ \left. \frac{1}{r^4} \left( 24 \vec{v}_1 \cdot \vec{v}_1 \vec{v}_1 \cdot \vec{v}_2 \left( \hat{n} \cdot \vec{S}_1 \right)^2 + 6 \vec{v}_1 \cdot \vec{v}_2 \vec{v}_2 \cdot \vec{v}_2 \left( \hat{n} \cdot \vec{S}_1 \right)^2 + 12 \vec{v}_1 \cdot \vec{v}_1 \hat{n} \cdot \vec{S}_1 \hat{n} \cdot \vec{v}_2 \vec{S}_1 \cdot \vec{v}_1 - \right. \right. \\ \left. \left. 16 \vec{v}_1 \cdot \vec{v}_1 \hat{n} \cdot \vec{S}_1 \hat{n} \cdot \vec{v}_1 \vec{S}_1 \cdot \vec{v}_2 - 8 \vec{v}_1 \cdot \vec{v}_2 \hat{n} \cdot \vec{S}_1 \hat{n} \cdot \vec{v}_1 \vec{S}_1 \cdot \vec{v}_1 + 4 \vec{v}_2 \cdot \vec{v}_2 \hat{n} \cdot \vec{S}_1 \hat{n} \cdot \vec{v}_2 \vec{S}_1 \cdot \vec{v}_1 - \right. \right. \\ \left. \left. 4 \vec{v}_2 \cdot \vec{v}_2 \hat{n} \cdot \vec{S}_1 \hat{n} \cdot \vec{v}_1 \vec{S}_1 \cdot \vec{v}_2 - 4 \hat{n} \cdot \vec{v}_1 \hat{n} \cdot \vec{v}_2 \left( \vec{S}_1 \cdot \vec{v}_1 \right)^2 + 4 \left( \hat{n} \cdot \vec{v}_1 \right)^2 \vec{S}_1 \cdot \vec{v}_1 \vec{S}_1 \cdot \vec{v}_2 + 8 \vec{S}_1 \cdot \vec{S}_1 \vec{v}_1 \cdot \vec{v}_1 \hat{n} \cdot \vec{v}_1 \hat{n} \cdot \vec{v}_2 + \right. \right. \\ \left. \left. 4 \vec{S}_1 \cdot \vec{S}_1 \vec{v}_1 \cdot \vec{v}_2 \left( \hat{n} \cdot \vec{v}_1 \right)^2 + 4 \vec{v}_1 \cdot \vec{v}_2 \left( \vec{S}_1 \cdot \vec{v}_1 \right)^2 - 12 \vec{S}_1 \cdot \vec{S}_1 \vec{v}_1 \cdot \vec{v}_1 \vec{v}_1 \cdot \vec{v}_2 - 2 \vec{S}_1 \cdot \vec{S}_1 \vec{v}_1 \cdot \vec{v}_2 \vec{v}_2 \cdot \vec{v}_2 \right) - \frac{8 \vec{S}_1^2 \vec{v}_1 \cdot \vec{v}_2}{r^2} \right) \Bigg\}$$

{DiagS1CES2[2, 2, 67],

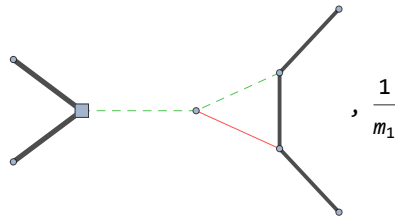

$$G^2 m_2^2 C_{ES^2 1} \left( \frac{1}{r^3} \left( -8 \vec{S}_1 \cdot \vec{S}_1 \vec{a}_1 \cdot \vec{v}_2 \hat{n} \cdot \vec{v}_1 + 8 \vec{S}_1 \cdot \vec{S}_1 \vec{v}_1 \cdot \vec{a}_1 \hat{n} \cdot \vec{v}_2 - 8 \vec{S}_1 \cdot \vec{S}_1 \vec{v}_1 \cdot \vec{v}_2 \hat{n} \cdot \vec{a}_1 + \right. \right. \\ \left. \left. 4 \vec{a}_1 \cdot \vec{v}_2 \hat{n} \cdot \vec{S}_1 \vec{S}_1 \cdot \vec{v}_1 + 4 \vec{S}_1 \cdot \vec{a}_1 \hat{n} \cdot \vec{v}_1 \vec{S}_1 \cdot \vec{v}_2 + 4 \hat{n} \cdot \vec{a}_1 \vec{S}_1 \cdot \vec{v}_1 \vec{S}_1 \cdot \vec{v}_2 - 8 \vec{v}_1 \cdot \vec{a}_1 \hat{n} \cdot \vec{S}_1 \vec{S}_1 \cdot \vec{v}_2 + \right. \right. \\ \left. \left. 4 \vec{v}_1 \cdot \vec{v}_2 \vec{S}_1 \cdot \vec{a}_1 \hat{n} \cdot \vec{S}_1 + 4 \hat{n} \cdot \vec{v}_1 \vec{S}_1 \cdot \vec{v}_2 \vec{S}_1 \cdot \vec{v}_1 + 4 \hat{n} \cdot \vec{v}_1 \vec{S}_1 \cdot \vec{v}_1 \vec{S}_1 \cdot \vec{v}_2 - 4 \vec{v}_1 \cdot \vec{v}_1 \hat{n} \cdot \vec{S}_1 \vec{S}_1 \cdot \vec{v}_2 + \right. \right. \\ \left. \left. 8 \vec{S}_1 \cdot \vec{S}_1 \vec{v}_1 \cdot \vec{v}_1 \hat{n} \cdot \vec{v}_2 - 4 \vec{v}_1 \cdot \vec{v}_1 \hat{n} \cdot \vec{S}_1 \vec{S}_1 \cdot \vec{v}_2 + 4 \vec{v}_1 \cdot \vec{v}_2 \hat{n} \cdot \vec{S}_1 \vec{S}_1 \cdot \vec{v}_1 - 16 \vec{S}_1 \cdot \vec{S}_1 \vec{v}_1 \cdot \vec{v}_2 \hat{n} \cdot \vec{v}_1 + \right. \right. \\ \left. \left. 8 \vec{S}_1 \cdot \vec{S}_1 \vec{v}_1 \cdot \vec{v}_2 \hat{n} \cdot \vec{v}_1 - 8 \vec{S}_1 \cdot \vec{S}_1 \vec{v}_1 \cdot \vec{v}_2 \hat{n} \cdot \vec{v}_1 \right) \right)$$

,  $\frac{1}{m_1}$

$$\begin{aligned}
& 4 \vec{v}_1 \cdot \vec{v}_2 \hat{n} \cdot \vec{S}_1 \vec{S}_1 \cdot \vec{v}_1 - 16 \vec{v}_2 \cdot \vec{v}_2 \hat{n} \cdot \vec{S}_1 \vec{S}_1 \cdot \vec{v}_2 + 32 \vec{S}_1 \cdot \vec{S}_1 \vec{v}_2 \cdot \vec{v}_2 \hat{n} \cdot \vec{v}_2 - 16 \vec{v}_2 \cdot \vec{v}_2 \hat{n} \cdot \vec{S}_1 \vec{S}_1 \cdot \vec{v}_2 \Big) + \\
& \frac{1}{r^4} \Big( 16 \vec{v}_1 \cdot \vec{v}_1 \vec{v}_1 \cdot \vec{v}_2 \left( \hat{n} \cdot \vec{S}_1 \right)^2 + 64 \vec{v}_1 \cdot \vec{v}_2 \vec{v}_2 \cdot \vec{v}_2 \left( \hat{n} \cdot \vec{S}_1 \right)^2 - 32 \vec{v}_1 \cdot \vec{v}_2 \hat{n} \cdot \vec{S}_1 \hat{n} \cdot \vec{v}_1 \vec{S}_1 \cdot \vec{v}_1 + \\
& 32 \vec{S}_1 \cdot \vec{S}_1 \vec{v}_1 \cdot \vec{v}_2 \left( \hat{n} \cdot \vec{v}_1 \right)^2 + 8 \vec{v}_1 \cdot \vec{v}_2 \left( \vec{S}_1 \cdot \vec{v}_1 \right)^2 - 16 \vec{S}_1 \cdot \vec{S}_1 \vec{v}_1 \cdot \vec{v}_1 \vec{v}_1 \cdot \vec{v}_2 - 32 \vec{S}_1 \cdot \vec{S}_1 \vec{v}_1 \cdot \vec{v}_2 \vec{v}_2 \cdot \vec{v}_2 \Big) \Big) \Big\}
\end{aligned}$$

$\{ \text{DiagS1CES2}[2, 2, 68],$ 
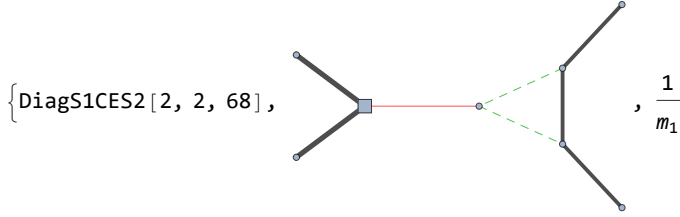
 $, \frac{1}{m_1}$

$$\begin{aligned}
& G^2 m_2^2 C_{\text{ES}^2} \left( \frac{8 \vec{v}_2 \cdot \vec{v}_2 \vec{S}_1 \cdot \vec{a}_1 \hat{n} \cdot \vec{S}_1 + 8 \vec{v}_2 \cdot \vec{v}_2 \hat{n} \cdot \vec{S}_1 \vec{S}_1 \cdot \vec{v}_1 - 16 \vec{S}_1 \cdot \vec{S}_1 \vec{v}_2 \cdot \vec{v}_2 \hat{n} \cdot \vec{v}_1 + 8 \vec{v}_2 \cdot \vec{v}_2 \hat{n} \cdot \vec{S}_1 \vec{S}_1 \cdot \vec{v}_1}{r^3} + \right. \\
& \frac{1}{r^4} \left( -16 \left( \vec{v}_2 \cdot \vec{v}_2 \right)^2 \left( \hat{n} \cdot \vec{S}_1 \right)^2 - 24 \vec{v}_1 \cdot \vec{v}_1 \vec{v}_2 \cdot \vec{v}_2 \left( \hat{n} \cdot \vec{S}_1 \right)^2 + 16 \vec{v}_2 \cdot \vec{v}_2 \hat{n} \cdot \vec{S}_1 \hat{n} \cdot \vec{v}_1 \vec{S}_1 \cdot \vec{v}_1 - \right. \\
& \left. \left. 16 \vec{S}_1 \cdot \vec{S}_1 \vec{v}_2 \cdot \vec{v}_2 \left( \hat{n} \cdot \vec{v}_1 \right)^2 + 8 \vec{S}_1 \cdot \vec{S}_1 \left( \vec{v}_2 \cdot \vec{v}_2 \right)^2 - 4 \vec{v}_2 \cdot \vec{v}_2 \left( \vec{S}_1 \cdot \vec{v}_1 \right)^2 + 16 \vec{S}_1 \cdot \vec{S}_1 \vec{v}_1 \cdot \vec{v}_1 \vec{v}_2 \cdot \vec{v}_2 \right) + \frac{4 \vec{S}_1^2 \vec{v}_2 \cdot \vec{v}_2}{r^2} \right) \Big\}
\end{aligned}$$

$\{ \text{DiagS1CES2}[2, 2, 69],$ 
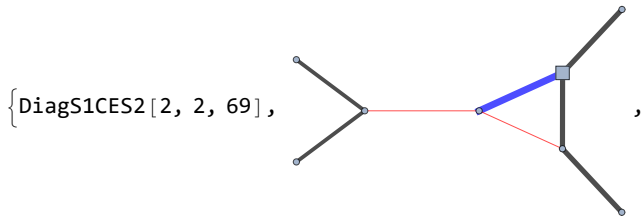
 $,$

$$\begin{aligned}
& G^2 \left( \frac{1}{r^2} \left( 8 \vec{v}_1 \cdot \vec{v}_1 \left( \hat{n} \cdot \vec{S}_1 \right)^2 + 6 \vec{v}_2 \cdot \vec{v}_2 \left( \hat{n} \cdot \vec{S}_1 \right)^2 - 4 \hat{n} \cdot \vec{v}_1 \vec{S}_1 \cdot \vec{v}_1 \hat{n} \cdot \vec{S}_1 - 4 \hat{n} \cdot \vec{v}_1 \vec{S}_1 \cdot \vec{a}_1 \hat{n} \cdot \vec{S}_1 - 4 \hat{n} \cdot \vec{a}_1 \vec{S}_1 \cdot \vec{v}_1 \hat{n} \cdot \vec{S}_1 + \right. \right. \\
& 8 \hat{n} \cdot \vec{S}_1 \vec{v}_1 \cdot \vec{a}_1 \hat{n} \cdot \vec{S}_1 + 2 \left( \vec{S}_1 \cdot \vec{v}_1 \right)^2 + 2 \left( \vec{S}_1 \cdot \vec{a}_1 \right)^2 + 4 \left( \hat{n} \cdot \vec{v}_1 \right)^2 \vec{S}_1 \cdot \vec{S}_1 + 8 \hat{n} \cdot \vec{v}_1 \hat{n} \cdot \vec{v}_2 \vec{S}_1 \cdot \vec{S}_1 - \\
& 4 \hat{n} \cdot \vec{S}_1 \hat{n} \cdot \vec{v}_1 \vec{S}_1 \cdot \vec{a}_1 - 4 \hat{n} \cdot \vec{a}_1 \hat{n} \cdot \vec{S}_1 \vec{S}_1 \cdot \vec{v}_1 - 2 \hat{n} \cdot \vec{S}_1 \hat{n} \cdot \vec{v}_1 \vec{S}_1 \cdot \vec{v}_1 + 2 \left( \hat{n} \cdot \vec{S}_1 \right)^2 \vec{a}_1 \cdot \vec{a}_1 - 2 \hat{n} \cdot \vec{S}_1 \hat{n} \cdot \vec{v}_1 \vec{S}_1 \cdot \vec{a}_1 + \\
& 16 \hat{n} \cdot \vec{a}_1 \hat{n} \cdot \vec{v}_1 \vec{S}_1 \cdot \vec{S}_1 + 4 \left( \hat{n} \cdot \vec{v}_1 \right)^2 \vec{S}_1 \cdot \vec{S}_1 + 8 \hat{n} \cdot \vec{v}_1 \hat{n} \cdot \vec{v}_2 \vec{S}_1 \cdot \vec{S}_1 - 4 \hat{n} \cdot \vec{a}_1 \hat{n} \cdot \vec{S}_1 \vec{S}_1 \cdot \vec{a}_1 + 4 \vec{S}_1 \cdot \vec{v}_1 \vec{S}_1 \cdot \vec{a}_1 + \\
& 4 \left( \hat{n} \cdot \vec{a}_1 \right)^2 \vec{S}_1 \cdot \vec{S}_1 + 4 \hat{n} \cdot \vec{a}_1 \hat{n} \cdot \vec{v}_1 \vec{S}_1 \cdot \vec{S}_1 - 2 \vec{a}_1 \cdot \vec{a}_1 \vec{S}_1 \cdot \vec{S}_1 - 2 \hat{n} \cdot \vec{a}_1 \hat{n} \cdot \vec{S}_1 \vec{S}_1 \cdot \vec{v}_1 - 2 \hat{n} \cdot \vec{S}_1 \hat{n} \cdot \vec{v}_1 \vec{S}_1 \cdot \vec{v}_1 + \\
& 4 \vec{S}_1 \cdot \vec{a}_1 \vec{S}_1 \cdot \vec{v}_1 + 2 \vec{S}_1 \cdot \vec{v}_1 \vec{S}_1 \cdot \vec{v}_1 + 2 \vec{S}_1 \cdot \vec{a}_1 \vec{S}_1 \cdot \vec{v}_1 + 2 \left( \hat{n} \cdot \vec{S}_1 \right)^2 \vec{v}_1 \cdot \vec{a}_1 - 2 \vec{S}_1 \cdot \vec{S}_1 \vec{v}_1 \cdot \vec{a}_1 - 8 \vec{S}_1 \cdot \vec{S}_1 \vec{v}_1 \cdot \vec{a}_1 + \\
& 8 \hat{n} \cdot \vec{S}_1 \hat{n} \cdot \vec{S}_1 \vec{v}_1 \cdot \vec{v}_1 - 2 \vec{S}_1 \cdot \vec{S}_1 \vec{v}_1 \cdot \vec{v}_1 - 2 \vec{S}_1 \cdot \vec{S}_1 \vec{v}_1 \cdot \vec{v}_1 - 4 \vec{S}_1 \cdot \vec{S}_1 \vec{v}_1 \cdot \vec{v}_2 - 4 \vec{S}_1 \cdot \vec{S}_1 \vec{v}_1 \cdot \vec{v}_2 + 6 \hat{n} \cdot \vec{S}_1 \hat{n} \cdot \vec{S}_1 \vec{v}_2 \cdot \vec{v}_2 \Big) + \\
& \frac{1}{r^3} \left( -8 \vec{S}_1 \cdot \vec{S}_1 \left( \hat{n} \cdot \vec{v}_1 \right)^3 + 4 \hat{n} \cdot \vec{S}_1 \vec{S}_1 \cdot \vec{v}_1 \left( \hat{n} \cdot \vec{v}_1 \right)^2 - 8 \hat{n} \cdot \vec{v}_2 \vec{S}_1 \cdot \vec{S}_1 \left( \hat{n} \cdot \vec{v}_1 \right)^2 + 4 \hat{n} \cdot \vec{S}_1 \vec{S}_1 \cdot \vec{a}_1 \left( \hat{n} \cdot \vec{v}_1 \right)^2 - \right. \\
& 10 \hat{n} \cdot \vec{a}_1 \vec{S}_1 \cdot \vec{S}_1 \left( \hat{n} \cdot \vec{v}_1 \right)^2 + 4 \hat{n} \cdot \vec{S}_1 \vec{S}_1 \cdot \vec{v}_1 \left( \hat{n} \cdot \vec{v}_1 \right)^2 + 4 \hat{n} \cdot \vec{S}_1 \hat{n} \cdot \vec{v}_2 \vec{S}_1 \cdot \vec{v}_1 \hat{n} \cdot \vec{v}_1 + 4 \hat{n} \cdot \vec{S}_1 \hat{n} \cdot \vec{v}_2 \vec{S}_1 \cdot \vec{a}_1 \hat{n} \cdot \vec{v}_1 + \\
& 6 \hat{n} \cdot \vec{a}_1 \hat{n} \cdot \vec{S}_1 \vec{S}_1 \cdot \vec{v}_1 \hat{n} \cdot \vec{v}_1 + 4 \hat{n} \cdot \vec{S}_1 \hat{n} \cdot \vec{v}_2 \vec{S}_1 \cdot \vec{v}_1 \hat{n} \cdot \vec{v}_1 - \frac{11}{2} \vec{S}_1 \cdot \vec{v}_1 \vec{S}_1 \cdot \vec{v}_1 \hat{n} \cdot \vec{v}_1 - \vec{S}_1 \cdot \vec{v}_2 \vec{S}_1 \cdot \vec{v}_1 \hat{n} \cdot \vec{v}_1 - \\
& \frac{19}{4} \vec{S}_1 \cdot \vec{a}_1 \vec{S}_1 \cdot \vec{v}_1 \hat{n} \cdot \vec{v}_1 - \vec{S}_1 \cdot \vec{v}_1 \vec{S}_1 \cdot \vec{v}_2 \hat{n} \cdot \vec{v}_1 - \vec{S}_1 \cdot \vec{a}_1 \vec{S}_1 \cdot \vec{v}_2 \hat{n} \cdot \vec{v}_1 - 4 \left( \hat{n} \cdot \vec{S}_1 \right)^2 \vec{v}_1 \cdot \vec{a}_1 \hat{n} \cdot \vec{v}_1 + \\
& 5 \vec{S}_1 \cdot \vec{S}_1 \vec{v}_1 \cdot \vec{a}_1 \hat{n} \cdot \vec{v}_1 - 16 \hat{n} \cdot \vec{S}_1 \hat{n} \cdot \vec{S}_1 \vec{v}_1 \cdot \vec{v}_1 \hat{n} \cdot \vec{v}_1 + 2 \vec{S}_1 \cdot \vec{S}_1 \vec{v}_1 \cdot \vec{v}_1 \hat{n} \cdot \vec{v}_1 + 4 \vec{S}_1 \cdot \vec{S}_1 \vec{v}_1 \cdot \vec{v}_2 \hat{n} \cdot \vec{v}_1 -
\end{aligned}$$

$$\begin{aligned}
& 12 \hat{n} \cdot \vec{S}_1 \hat{n} \cdot \vec{S}_1 \vec{v}_2 \cdot \vec{v}_2 \hat{n} \cdot \vec{v}_1 - \frac{9}{2} \vec{S}_1 \cdot \vec{S}_1 \vec{v}_2 \cdot \vec{v}_2 \hat{n} \cdot \vec{v}_1 - \frac{9}{4} \hat{n} \cdot \vec{a}_1 \left( \vec{S}_1 \cdot \vec{v}_1 \right)^2 - 4 \hat{n} \cdot \vec{v}_2 \vec{S}_1 \cdot \vec{v}_1 \vec{S}_1 \cdot \vec{v}_1 - \\
& 2 \hat{n} \cdot \vec{v}_2 \vec{S}_1 \cdot \vec{a}_1 \vec{S}_1 \cdot \vec{v}_1 + \frac{3}{4} \hat{n} \cdot \vec{S}_1 \vec{S}_1 \cdot \vec{v}_1 \vec{v}_1 \cdot \vec{a}_1 - 4 \hat{n} \cdot \vec{a}_1 \left( \hat{n} \cdot \vec{S}_1 \right)^2 \vec{v}_1 \cdot \vec{v}_1 + \frac{15}{4} \hat{n} \cdot \vec{S}_1 \vec{S}_1 \cdot \vec{v}_1 \vec{v}_1 \cdot \vec{v}_1 + \\
& 4 \hat{n} \cdot \vec{v}_2 \vec{S}_1 \cdot \vec{S}_1 \vec{v}_1 \cdot \vec{v}_1 + \frac{3}{4} \hat{n} \cdot \vec{S}_1 \vec{S}_1 \cdot \vec{a}_1 \vec{v}_1 \cdot \vec{v}_1 + \frac{3}{2} \hat{n} \cdot \vec{a}_1 \vec{S}_1 \cdot \vec{S}_1 \vec{v}_1 \cdot \vec{v}_1 + \frac{15}{4} \hat{n} \cdot \vec{S}_1 \vec{S}_1 \cdot \vec{v}_1 \vec{v}_1 \cdot \vec{v}_1 - \\
& \hat{n} \cdot \vec{S}_1 \vec{S}_1 \cdot \vec{v}_1 \vec{v}_1 \cdot \vec{v}_2 - \hat{n} \cdot \vec{S}_1 \vec{S}_1 \cdot \vec{a}_1 \vec{v}_1 \cdot \vec{v}_2 - \hat{n} \cdot \vec{S}_1 \vec{S}_1 \cdot \vec{v}_1 \vec{v}_1 \cdot \vec{v}_2 - 3 \hat{n} \cdot \vec{a}_1 \left( \hat{n} \cdot \vec{S}_1 \right)^2 \vec{v}_2 \cdot \vec{v}_2 + \\
& \frac{15}{4} \hat{n} \cdot \vec{S}_1 \vec{S}_1 \cdot \vec{v}_1 \vec{v}_2 \cdot \vec{v}_2 + \frac{3}{2} \hat{n} \cdot \vec{S}_1 \vec{S}_1 \cdot \vec{a}_1 \vec{v}_2 \cdot \vec{v}_2 - \frac{3}{2} \hat{n} \cdot \vec{a}_1 \vec{S}_1 \cdot \vec{S}_1 \vec{v}_2 \cdot \vec{v}_2 + \frac{15}{4} \hat{n} \cdot \vec{S}_1 \vec{S}_1 \cdot \vec{v}_1 \vec{v}_2 \cdot \vec{v}_2 \Big) + \frac{1}{r^4} \\
& \left( 6 \vec{S}_1 \cdot \vec{S}_1 \left( \hat{n} \cdot \vec{v}_1 \right)^4 - 6 \hat{n} \cdot \vec{S}_1 \vec{S}_1 \cdot \vec{v}_1 \left( \hat{n} \cdot \vec{v}_1 \right)^3 + 3 \left( \vec{S}_1 \cdot \vec{v}_1 \right)^2 \left( \hat{n} \cdot \vec{v}_1 \right)^2 + 12 \left( \hat{n} \cdot \vec{S}_1 \right)^2 \vec{v}_1 \cdot \vec{v}_1 \left( \hat{n} \cdot \vec{v}_1 \right)^2 - \right. \\
& 7 \vec{S}_1 \cdot \vec{S}_1 \vec{v}_1 \cdot \vec{v}_1 \left( \hat{n} \cdot \vec{v}_1 \right)^2 + 9 \left( \hat{n} \cdot \vec{S}_1 \right)^2 \vec{v}_2 \cdot \vec{v}_2 \left( \hat{n} \cdot \vec{v}_1 \right)^2 - 6 \left( \hat{n} \cdot \vec{S}_1 \right)^2 \hat{n} \cdot \vec{v}_2 \vec{v}_1 \cdot \vec{v}_1 \hat{n} \cdot \vec{v}_1 - \\
& 8 \hat{n} \cdot \vec{S}_1 \vec{S}_1 \cdot \vec{v}_1 \vec{v}_1 \cdot \vec{v}_1 \hat{n} \cdot \vec{v}_1 + 2 \hat{n} \cdot \vec{S}_1 \vec{S}_1 \cdot \vec{v}_2 \vec{v}_1 \cdot \vec{v}_1 \hat{n} \cdot \vec{v}_1 - 9 \hat{n} \cdot \vec{S}_1 \vec{S}_1 \cdot \vec{v}_1 \vec{v}_2 \cdot \vec{v}_2 \hat{n} \cdot \vec{v}_1 - \\
& 2 \left( \hat{n} \cdot \vec{S}_1 \right)^2 \left( \vec{v}_1 \cdot \vec{v}_1 \right)^2 + \vec{S}_1 \cdot \vec{S}_1 \left( \vec{v}_1 \cdot \vec{v}_1 \right)^2 + \left( \vec{S}_1 \cdot \vec{v}_1 \right)^2 \vec{v}_1 \cdot \vec{v}_1 + 4 \hat{n} \cdot \vec{S}_1 \hat{n} \cdot \vec{v}_2 \vec{S}_1 \cdot \vec{v}_1 \vec{v}_1 \cdot \vec{v}_1 - \\
& \left. \vec{S}_1 \cdot \vec{v}_1 \vec{S}_1 \cdot \vec{v}_2 \vec{v}_1 \cdot \vec{v}_1 + \left( \hat{n} \cdot \vec{S}_1 \right)^2 \vec{v}_1 \cdot \vec{v}_1 \vec{v}_1 \cdot \vec{v}_2 + \frac{3}{2} \left( \vec{S}_1 \cdot \vec{v}_1 \right)^2 \vec{v}_2 \cdot \vec{v}_2 - \frac{3}{2} \left( \hat{n} \cdot \vec{S}_1 \right)^2 \vec{v}_1 \cdot \vec{v}_1 \vec{v}_2 \cdot \vec{v}_2 \right) \Big) m_2 C_{ES^2 1} \Big\}
\end{aligned}$$

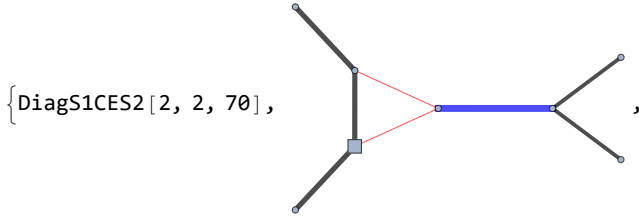

$$\begin{aligned}
& G^2 \left( \frac{1}{r^3} \left( 2 \hat{n} \cdot \vec{S}_1 \vec{S}_1 \cdot \vec{v}_1 \left( \hat{n} \cdot \vec{v}_2 \right)^2 - 4 \hat{n} \cdot \vec{v}_1 \vec{S}_1 \cdot \vec{S}_1 \left( \hat{n} \cdot \vec{v}_2 \right)^2 + 2 \hat{n} \cdot \vec{S}_1 \vec{S}_1 \cdot \vec{a}_1 \left( \hat{n} \cdot \vec{v}_2 \right)^2 + \right. \right. \\
& 2 \hat{n} \cdot \vec{S}_1 \vec{S}_1 \cdot \vec{v}_1 \left( \hat{n} \cdot \vec{v}_2 \right)^2 - \vec{S}_1 \cdot \vec{v}_2 \vec{S}_1 \cdot \vec{v}_1 \hat{n} \cdot \vec{v}_2 - \vec{S}_1 \cdot \vec{v}_1 \vec{S}_1 \cdot \vec{v}_2 \hat{n} \cdot \vec{v}_2 - \vec{S}_1 \cdot \vec{a}_1 \vec{S}_1 \cdot \vec{v}_2 \hat{n} \cdot \vec{v}_2 + \\
& \left. 2 \vec{S}_1 \cdot \vec{S}_1 \vec{v}_1 \cdot \vec{v}_2 \hat{n} \cdot \vec{v}_2 - 2 \hat{n} \cdot \vec{S}_1 \hat{n} \cdot \vec{S}_1 \hat{n} \cdot \vec{v}_1 \vec{v}_2 \cdot \vec{v}_2 + 2 \hat{n} \cdot \vec{v}_1 \vec{S}_1 \cdot \vec{S}_1 \vec{v}_2 \cdot \vec{v}_2 - \hat{n} \cdot \vec{S}_1 \vec{S}_1 \cdot \vec{a}_1 \vec{v}_2 \cdot \vec{v}_2 \right) + \\
& \frac{1}{r^4} \left( \frac{5}{8} \left( \vec{v}_2 \cdot \vec{v}_2 \right)^2 \left( \hat{n} \cdot \vec{S}_1 \right)^2 - \frac{45}{4} \left( \hat{n} \cdot \vec{v}_2 \right)^2 \vec{v}_1 \cdot \vec{v}_1 \left( \hat{n} \cdot \vec{S}_1 \right)^2 + \frac{15}{4} \left( \hat{n} \cdot \vec{v}_1 \right)^2 \vec{v}_2 \cdot \vec{v}_2 \left( \hat{n} \cdot \vec{S}_1 \right)^2 - \right. \\
& \frac{15}{8} \left( \hat{n} \cdot \vec{v}_2 \right)^2 \vec{v}_2 \cdot \vec{v}_2 \left( \hat{n} \cdot \vec{S}_1 \right)^2 + \frac{5}{2} \vec{v}_1 \cdot \vec{v}_1 \vec{v}_2 \cdot \vec{v}_2 \left( \hat{n} \cdot \vec{S}_1 \right)^2 + \frac{15}{4} \hat{n} \cdot \vec{v}_1 \left( \hat{n} \cdot \vec{v}_2 \right)^2 \vec{S}_1 \cdot \vec{v}_1 \hat{n} \cdot \vec{S}_1 + \\
& 9 \hat{n} \cdot \vec{v}_2 \vec{S}_1 \cdot \vec{v}_2 \vec{v}_1 \cdot \vec{v}_1 \hat{n} \cdot \vec{S}_1 - \frac{3}{2} \hat{n} \cdot \vec{v}_2 \vec{S}_1 \cdot \vec{v}_1 \vec{v}_1 \cdot \vec{v}_2 \hat{n} \cdot \vec{S}_1 - \frac{17}{4} \hat{n} \cdot \vec{v}_1 \vec{S}_1 \cdot \vec{v}_1 \vec{v}_2 \cdot \vec{v}_2 \hat{n} \cdot \vec{S}_1 + \\
& \frac{3}{2} \hat{n} \cdot \vec{v}_2 \vec{S}_1 \cdot \vec{v}_2 \vec{v}_2 \cdot \vec{v}_2 \hat{n} \cdot \vec{S}_1 - \frac{1}{4} \left( \hat{n} \cdot \vec{v}_2 \right)^2 \left( \vec{S}_1 \cdot \vec{v}_1 \right)^2 - \frac{1}{2} \vec{S}_1 \cdot \vec{S}_1 \left( \vec{v}_1 \cdot \vec{v}_2 \right)^2 - \frac{1}{8} \vec{S}_1 \cdot \vec{S}_1 \left( \vec{v}_2 \cdot \vec{v}_2 \right)^2 - \\
& \frac{15}{4} \left( \hat{n} \cdot \vec{v}_1 \right)^2 \left( \hat{n} \cdot \vec{v}_2 \right)^2 \vec{S}_1 \cdot \vec{S}_1 - \frac{3}{2} \hat{n} \cdot \vec{v}_1 \hat{n} \cdot \vec{v}_2 \vec{S}_1 \cdot \vec{v}_1 \vec{S}_1 \cdot \vec{v}_2 - \frac{3}{2} \left( \vec{S}_1 \cdot \vec{v}_2 \right)^2 \vec{v}_1 \cdot \vec{v}_1 + \left( \hat{n} \cdot \vec{v}_2 \right)^2 \vec{S}_1 \cdot \vec{S}_1 \vec{v}_1 \cdot \vec{v}_1 + \\
& 3 \hat{n} \cdot \vec{v}_1 \hat{n} \cdot \vec{v}_2 \vec{S}_1 \cdot \vec{S}_1 \vec{v}_1 \cdot \vec{v}_2 + \frac{1}{2} \vec{S}_1 \cdot \vec{v}_1 \vec{S}_1 \cdot \vec{v}_2 \vec{v}_1 \cdot \vec{v}_2 + \frac{3}{4} \left( \vec{S}_1 \cdot \vec{v}_1 \right)^2 \vec{v}_2 \cdot \vec{v}_2 - \frac{1}{4} \left( \vec{S}_1 \cdot \vec{v}_2 \right)^2 \vec{v}_2 \cdot \vec{v}_2 + \\
& \left. \left( \hat{n} \cdot \vec{v}_1 \right)^2 \vec{S}_1 \cdot \vec{S}_1 \vec{v}_2 \cdot \vec{v}_2 + \frac{1}{8} \left( \hat{n} \cdot \vec{v}_2 \right)^2 \vec{S}_1 \cdot \vec{S}_1 \vec{v}_2 \cdot \vec{v}_2 - \frac{3}{4} \vec{S}_1 \cdot \vec{S}_1 \vec{v}_1 \cdot \vec{v}_1 \vec{v}_2 \cdot \vec{v}_2 \right) + \frac{\left( \hat{n} \cdot \vec{v}_2 \right)^2 \vec{S}_1^2 - \vec{v}_2 \cdot \vec{v}_2 \vec{S}_1^2}{r^2} \Big) m_2 C_{ES^2 1} \Big\}
\end{aligned}$$

{DiagS1CES2[2, 2, 71],

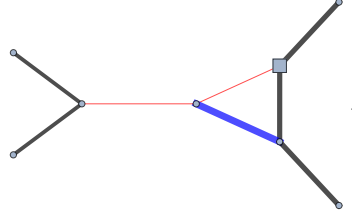

,

$$\begin{aligned}
 G^2 \left( \frac{1}{r^3} \left( 24 \vec{S}_1 \cdot \vec{S}_1 (\hat{n} \cdot \vec{v}_1)^3 - 12 \hat{n} \cdot \vec{S}_1 \vec{S}_1 \cdot \vec{v}_1 (\hat{n} \cdot \vec{v}_1)^2 - 12 \hat{n} \cdot \vec{S}_1 \vec{S}_1 \cdot \vec{a}_1 (\hat{n} \cdot \vec{v}_1)^2 - \right. \right. \\
 12 \hat{n} \cdot \vec{S}_1 \vec{S}_1 \cdot \vec{v}_1 (\hat{n} \cdot \vec{v}_1)^2 + 10 \vec{S}_1 \cdot \vec{v}_1 \vec{S}_1 \cdot \vec{v}_1 \hat{n} \cdot \vec{v}_1 + 5 \vec{S}_1 \cdot \vec{a}_1 \vec{S}_1 \cdot \vec{v}_1 \hat{n} \cdot \vec{v}_1 - 16 \vec{S}_1 \cdot \vec{S}_1 \vec{v}_1 \cdot \vec{v}_1 \hat{n} \cdot \vec{v}_1 + \\
 12 \hat{n} \cdot \vec{S}_1 \hat{n} \cdot \vec{S}_1 \hat{n} \cdot \vec{v}_2 \vec{v}_1 \cdot \vec{v}_1 + 3 \hat{n} \cdot \vec{S}_1 \vec{S}_1 \cdot \vec{v}_1 \vec{v}_1 \cdot \vec{v}_1 - 3 \hat{n} \cdot \vec{S}_1 \vec{S}_1 \cdot \vec{v}_2 \vec{v}_1 \cdot \vec{v}_1 - \\
 \left. \left. 2 \hat{n} \cdot \vec{v}_2 \vec{S}_1 \cdot \vec{S}_1 \vec{v}_1 \cdot \vec{v}_1 + 3 \hat{n} \cdot \vec{S}_1 \vec{S}_1 \cdot \vec{a}_1 \vec{v}_1 \cdot \vec{v}_1 + 3 \hat{n} \cdot \vec{S}_1 \vec{S}_1 \cdot \vec{v}_1 \vec{v}_1 \cdot \vec{v}_1 - 3 \hat{n} \cdot \vec{S}_1 \vec{S}_1 \cdot \vec{v}_2 \vec{v}_1 \cdot \vec{v}_1 \right) + \frac{1}{r^4} \right. \\
 \left( 30 \vec{S}_1 \cdot \vec{S}_1 (\hat{n} \cdot \vec{v}_1)^4 - 30 \hat{n} \cdot \vec{S}_1 \vec{S}_1 \cdot \vec{v}_1 (\hat{n} \cdot \vec{v}_1)^3 + 13 (\vec{S}_1 \cdot \vec{v}_1)^2 (\hat{n} \cdot \vec{v}_1)^2 + 60 (\hat{n} \cdot \vec{S}_1)^2 \vec{v}_1 \cdot \vec{v}_1 (\hat{n} \cdot \vec{v}_1)^2 - \right. \\
 35 \vec{S}_1 \cdot \vec{S}_1 \vec{v}_1 \cdot \vec{v}_1 (\hat{n} \cdot \vec{v}_1)^2 + 45 (\hat{n} \cdot \vec{S}_1)^2 \vec{v}_2 \cdot \vec{v}_2 (\hat{n} \cdot \vec{v}_1)^2 - 6 \vec{S}_1 \cdot \vec{S}_1 \vec{v}_2 \cdot \vec{v}_2 (\hat{n} \cdot \vec{v}_1)^2 - 30 (\hat{n} \cdot \vec{S}_1)^2 \hat{n} \cdot \vec{v}_2 \\
 \vec{v}_1 \cdot \vec{v}_1 \hat{n} \cdot \vec{v}_1 + 4 \hat{n} \cdot \vec{v}_2 \vec{S}_1 \cdot \vec{S}_1 \vec{v}_1 \cdot \vec{v}_1 \hat{n} \cdot \vec{v}_1 - 22 \hat{n} \cdot \vec{S}_1 \vec{S}_1 \cdot \vec{v}_1 \vec{v}_1 \cdot \vec{v}_1 \hat{n} \cdot \vec{v}_1 + 10 \hat{n} \cdot \vec{S}_1 \vec{S}_1 \cdot \vec{v}_2 \vec{v}_1 \cdot \vec{v}_1 \hat{n} \cdot \vec{v}_1 - \\
 27 \hat{n} \cdot \vec{S}_1 \vec{S}_1 \cdot \vec{v}_1 \vec{v}_2 \cdot \vec{v}_2 \hat{n} \cdot \vec{v}_1 - 10 (\hat{n} \cdot \vec{S}_1)^2 (\vec{v}_1 \cdot \vec{v}_1)^2 + 5 \vec{S}_1 \cdot \vec{S}_1 (\vec{v}_1 \cdot \vec{v}_1)^2 + (\vec{S}_1 \cdot \vec{v}_1)^2 \vec{v}_1 \cdot \vec{v}_1 + \\
 8 \hat{n} \cdot \vec{S}_1 \hat{n} \cdot \vec{v}_2 \vec{S}_1 \cdot \vec{v}_1 \vec{v}_1 \cdot \vec{v}_1 - 2 \vec{S}_1 \cdot \vec{v}_1 \vec{S}_1 \cdot \vec{v}_2 \vec{v}_1 \cdot \vec{v}_1 + 5 (\hat{n} \cdot \vec{S}_1)^2 \vec{v}_1 \cdot \vec{v}_1 \vec{v}_1 \cdot \vec{v}_2 - \vec{S}_1 \cdot \vec{S}_1 \vec{v}_1 \cdot \vec{v}_1 \vec{v}_1 \cdot \vec{v}_2 + \\
 \left. \left. 3 (\vec{S}_1 \cdot \vec{v}_1)^2 \vec{v}_2 \cdot \vec{v}_2 - \frac{15}{2} (\hat{n} \cdot \vec{S}_1)^2 \vec{v}_1 \cdot \vec{v}_1 \vec{v}_2 \cdot \vec{v}_2 + \frac{3}{2} \vec{S}_1 \cdot \vec{S}_1 \vec{v}_1 \cdot \vec{v}_1 \vec{v}_2 \cdot \vec{v}_2 \right) + \frac{2 \vec{v}_1 \cdot \vec{v}_1 \vec{S}_1^2 - 4 (\hat{n} \cdot \vec{v}_1)^2 \vec{S}_1^2}{r^2} \right) m_2 C_{ES^2 1} \}
 \end{aligned}$$

{DiagS1CES2[2, 2, 72],

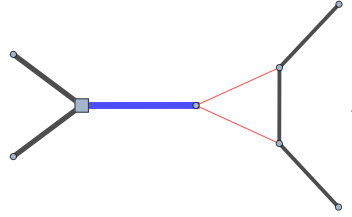

,  $\frac{1}{m_1}$

$$\begin{aligned}
 G^2 \left( \frac{1}{r^2} \left( -\frac{1}{4} \vec{v}_1 \cdot \vec{v}_1 (\hat{n} \cdot \vec{S}_1)^2 - \frac{3}{2} \vec{v}_2 \cdot \vec{v}_2 (\hat{n} \cdot \vec{S}_1)^2 + \frac{1}{2} \hat{n} \cdot \vec{v}_1 \vec{S}_1 \cdot \vec{v}_1 \hat{n} \cdot \vec{S}_1 + \frac{1}{2} \hat{n} \cdot \vec{v}_1 \vec{S}_1 \cdot \vec{a}_1 \hat{n} \cdot \vec{S}_1 + \frac{1}{2} \hat{n} \cdot \vec{a}_1 \vec{S}_1 \cdot \vec{v}_1 \hat{n} \cdot \vec{S}_1 - \right. \right. \\
 \hat{n} \cdot \vec{S}_1 \vec{v}_1 \cdot \vec{a}_1 \hat{n} \cdot \vec{S}_1 - \frac{1}{2} (\vec{S}_1 \cdot \vec{v}_1)^2 - \frac{1}{2} (\vec{S}_1 \cdot \vec{a}_1)^2 - \frac{1}{2} (\hat{n} \cdot \vec{v}_1)^2 \vec{S}_1 \cdot \vec{S}_1 - (\hat{n} \cdot \vec{v}_2)^2 \vec{S}_1 \cdot \vec{S}_1 + \frac{1}{2} \hat{n} \cdot \vec{S}_1 \hat{n} \cdot \vec{v}_1 \vec{S}_1 \cdot \vec{a}_1 + \\
 \frac{1}{2} \hat{n} \cdot \vec{a}_1 \hat{n} \cdot \vec{S}_1 \vec{S}_1 \cdot \vec{v}_1 + \frac{1}{4} \hat{n} \cdot \vec{S}_1 \hat{n} \cdot \vec{v}_1 \vec{S}_1 \cdot \vec{v}_1 - \frac{1}{4} (\hat{n} \cdot \vec{S}_1)^2 \vec{a}_1 \cdot \vec{a}_1 + \frac{1}{4} \hat{n} \cdot \vec{S}_1 \hat{n} \cdot \vec{v}_1 \vec{S}_1 \cdot \vec{a}_1 - 2 \hat{n} \cdot \vec{a}_1 \hat{n} \cdot \vec{v}_1 \vec{S}_1 \cdot \vec{S}_1 - \\
 \frac{1}{2} (\hat{n} \cdot \vec{v}_1)^2 \vec{S}_1 \cdot \vec{S}_1 - (\hat{n} \cdot \vec{v}_2)^2 \vec{S}_1 \cdot \vec{S}_1 + \frac{1}{2} \hat{n} \cdot \vec{a}_1 \hat{n} \cdot \vec{S}_1 \vec{S}_1 \cdot \vec{a}_1 - \vec{S}_1 \cdot \vec{v}_1 \vec{S}_1 \cdot \vec{a}_1 - \frac{1}{2} (\hat{n} \cdot \vec{a}_1)^2 \vec{S}_1 \cdot \vec{S}_1 - \\
 \frac{1}{2} \hat{n} \cdot \vec{a}_1 \hat{n} \cdot \vec{v}_1 \vec{S}_1 \cdot \vec{S}_1 + \frac{1}{4} \vec{a}_1 \cdot \vec{a}_1 \vec{S}_1 \cdot \vec{S}_1 + \frac{1}{4} \hat{n} \cdot \vec{a}_1 \hat{n} \cdot \vec{S}_1 \vec{S}_1 \cdot \vec{v}_1 + \frac{1}{4} \hat{n} \cdot \vec{S}_1 \hat{n} \cdot \vec{v}_1 \vec{S}_1 \cdot \vec{v}_1 - \vec{S}_1 \cdot \vec{a}_1 \vec{S}_1 \cdot \vec{v}_1 - \\
 \frac{1}{2} \vec{S}_1 \cdot \vec{v}_1 \vec{S}_1 \cdot \vec{v}_1 - \frac{1}{2} \vec{S}_1 \cdot \vec{a}_1 \vec{S}_1 \cdot \vec{v}_1 - \frac{1}{4} (\hat{n} \cdot \vec{S}_1)^2 \vec{v}_1 \cdot \vec{a}_1 + \frac{1}{4} \vec{S}_1 \cdot \vec{S}_1 \vec{v}_1 \cdot \vec{a}_1 + \vec{S}_1 \cdot \vec{S}_1 \vec{v}_1 \cdot \vec{a}_1 - \frac{1}{4} \hat{n} \cdot \vec{S}_1 \hat{n} \cdot \vec{S}_1 \vec{v}_1 \cdot \vec{v}_1 + \\
 \left. \left. \frac{1}{4} \vec{S}_1 \cdot \vec{S}_1 \vec{v}_1 \cdot \vec{v}_1 + \frac{1}{4} \vec{S}_1 \cdot \vec{S}_1 \vec{v}_1 \cdot \vec{v}_1 - \frac{3}{2} \hat{n} \cdot \vec{S}_1 \hat{n} \cdot \vec{S}_1 \vec{v}_2 \cdot \vec{v}_2 - \frac{1}{2} \vec{S}_1 \cdot \vec{S}_1 \vec{v}_2 \cdot \vec{v}_2 - \frac{1}{2} \vec{S}_1 \cdot \vec{S}_1 \vec{v}_2 \cdot \vec{v}_2 \right) + \frac{1}{r^3} \right. \\
 \left( 4 \vec{S}_1 \cdot \vec{S}_1 (\hat{n} \cdot \vec{v}_1)^3 - 2 \hat{n} \cdot \vec{S}_1 \vec{S}_1 \cdot \vec{v}_1 (\hat{n} \cdot \vec{v}_1)^2 - 2 \hat{n} \cdot \vec{S}_1 \vec{S}_1 \cdot \vec{a}_1 (\hat{n} \cdot \vec{v}_1)^2 + 5 \hat{n} \cdot \vec{a}_1 \vec{S}_1 \cdot \vec{S}_1 (\hat{n} \cdot \vec{v}_1)^2 - \right. \\
 \left. 2 \hat{n} \cdot \vec{S}_1 \vec{S}_1 \cdot \vec{v}_1 (\hat{n} \cdot \vec{v}_1)^2 + 4 (\hat{n} \cdot \vec{v}_2)^2 \vec{S}_1 \cdot \vec{S}_1 \hat{n} \cdot \vec{v}_1 - 3 \hat{n} \cdot \vec{a}_1 \hat{n} \cdot \vec{S}_1 \vec{S}_1 \cdot \vec{v}_1 \hat{n} \cdot \vec{v}_1 + \right.
 \end{aligned}$$

$$\begin{aligned}
& \frac{5}{2} \vec{S}_1 \cdot \vec{v}_1 \vec{S}_1 \cdot \vec{v}_1 \hat{n} \cdot \vec{v}_1 + \frac{9}{4} \vec{S}_1 \cdot \vec{a}_1 \vec{S}_1 \cdot \vec{v}_1 \hat{n} \cdot \vec{v}_1 + 2 \left( \hat{n} \cdot \vec{S}_1 \right)^2 \vec{v}_1 \cdot \vec{a}_1 \hat{n} \cdot \vec{v}_1 - 3 \vec{S}_1 \cdot \vec{S}_1 \vec{v}_1 \cdot \vec{a}_1 \hat{n} \cdot \vec{v}_1 + \\
& 2 \hat{n} \cdot \vec{S}_1 \hat{n} \cdot \vec{S}_1 \vec{v}_1 \cdot \vec{v}_1 \hat{n} \cdot \vec{v}_1 - \frac{7}{2} \vec{S}_1 \cdot \vec{S}_1 \vec{v}_1 \cdot \vec{v}_1 \hat{n} \cdot \vec{v}_1 + 12 \hat{n} \cdot \vec{S}_1 \hat{n} \cdot \vec{S}_1 \vec{v}_2 \cdot \vec{v}_2 \hat{n} \cdot \vec{v}_1 + \vec{S}_1 \cdot \vec{S}_1 \vec{v}_2 \cdot \vec{v}_2 \hat{n} \cdot \vec{v}_1 + \\
& \frac{3}{4} \hat{n} \cdot \vec{a}_1 \left( \vec{S}_1 \cdot \vec{v}_1 \right)^2 - 2 \hat{n} \cdot \vec{S}_1 \left( \hat{n} \cdot \vec{v}_2 \right)^2 \vec{S}_1 \cdot \vec{v}_1 - 2 \hat{n} \cdot \vec{S}_1 \left( \hat{n} \cdot \vec{v}_2 \right)^2 \vec{S}_1 \cdot \vec{a}_1 - 2 \hat{n} \cdot \vec{S}_1 \left( \hat{n} \cdot \vec{v}_2 \right)^2 \vec{S}_1 \cdot \vec{v}_1 + \\
& \hat{n} \cdot \vec{v}_2 \vec{S}_1 \cdot \vec{v}_2 \vec{S}_1 \cdot \vec{v}_1 + \hat{n} \cdot \vec{v}_2 \vec{S}_1 \cdot \vec{v}_1 \vec{S}_1 \cdot \vec{v}_2 + \hat{n} \cdot \vec{v}_2 \vec{S}_1 \cdot \vec{a}_1 \vec{S}_1 \cdot \vec{v}_2 - \frac{1}{4} \hat{n} \cdot \vec{S}_1 \vec{S}_1 \cdot \vec{v}_1 \vec{v}_1 \cdot \vec{a}_1 + \\
& \frac{1}{2} \hat{n} \cdot \vec{a}_1 \left( \hat{n} \cdot \vec{S}_1 \right)^2 \vec{v}_1 \cdot \vec{v}_1 + \frac{1}{4} \hat{n} \cdot \vec{S}_1 \vec{S}_1 \cdot \vec{a}_1 \vec{v}_1 \cdot \vec{v}_1 - \frac{3}{2} \hat{n} \cdot \vec{a}_1 \vec{S}_1 \cdot \vec{S}_1 \vec{v}_1 \cdot \vec{v}_1 - 2 \hat{n} \cdot \vec{v}_2 \vec{S}_1 \cdot \vec{S}_1 \vec{v}_1 \cdot \vec{v}_2 + \\
& 3 \hat{n} \cdot \vec{a}_1 \left( \hat{n} \cdot \vec{S}_1 \right)^2 \vec{v}_2 \cdot \vec{v}_2 - \frac{7}{2} \hat{n} \cdot \vec{S}_1 \vec{S}_1 \cdot \vec{v}_1 \vec{v}_2 \cdot \vec{v}_2 - 2 \hat{n} \cdot \vec{S}_1 \vec{S}_1 \cdot \vec{a}_1 \vec{v}_2 \cdot \vec{v}_2 - \frac{7}{2} \hat{n} \cdot \vec{S}_1 \vec{S}_1 \cdot \vec{v}_1 \vec{v}_2 \cdot \vec{v}_2 \Big) + \frac{1}{r^4} \\
& \left( -6 \vec{S}_1 \cdot \vec{S}_1 \left( \hat{n} \cdot \vec{v}_1 \right)^4 + 6 \hat{n} \cdot \vec{S}_1 \vec{S}_1 \cdot \vec{v}_1 \left( \hat{n} \cdot \vec{v}_1 \right)^3 - 3 \left( \vec{S}_1 \cdot \vec{v}_1 \right)^2 \left( \hat{n} \cdot \vec{v}_1 \right)^2 - 3 \left( \hat{n} \cdot \vec{S}_1 \right)^2 \vec{v}_1 \cdot \vec{v}_1 \left( \hat{n} \cdot \vec{v}_1 \right)^2 + \right. \\
& 7 \vec{S}_1 \cdot \vec{S}_1 \vec{v}_1 \cdot \vec{v}_1 \left( \hat{n} \cdot \vec{v}_1 \right)^2 - 18 \left( \hat{n} \cdot \vec{S}_1 \right)^2 \vec{v}_2 \cdot \vec{v}_2 \left( \hat{n} \cdot \vec{v}_1 \right)^2 - 2 \hat{n} \cdot \vec{S}_1 \vec{S}_1 \cdot \vec{v}_1 \vec{v}_1 \cdot \vec{v}_1 \hat{n} \cdot \vec{v}_1 + \\
& 12 \hat{n} \cdot \vec{S}_1 \vec{S}_1 \cdot \vec{v}_1 \vec{v}_2 \cdot \vec{v}_2 \hat{n} \cdot \vec{v}_1 + \left( \hat{n} \cdot \vec{S}_1 \right)^2 \left( \vec{v}_1 \cdot \vec{v}_1 \right)^2 - \frac{5}{4} \vec{S}_1 \cdot \vec{S}_1 \left( \vec{v}_1 \cdot \vec{v}_1 \right)^2 + \\
& 6 \left( \hat{n} \cdot \vec{S}_1 \right)^2 \left( \hat{n} \cdot \vec{v}_2 \right)^2 \vec{v}_1 \cdot \vec{v}_1 + \frac{3}{4} \left( \vec{S}_1 \cdot \vec{v}_1 \right)^2 \vec{v}_1 \cdot \vec{v}_1 + \frac{1}{2} \left( \vec{S}_1 \cdot \vec{v}_2 \right)^2 \vec{v}_1 \cdot \vec{v}_1 - 4 \hat{n} \cdot \vec{S}_1 \hat{n} \cdot \vec{v}_2 \vec{S}_1 \cdot \vec{v}_2 \vec{v}_1 \cdot \vec{v}_1 - \\
& \left. \frac{3}{2} \left( \vec{S}_1 \cdot \vec{v}_1 \right)^2 \vec{v}_2 \cdot \vec{v}_2 + 4 \left( \hat{n} \cdot \vec{S}_1 \right)^2 \vec{v}_1 \cdot \vec{v}_1 \vec{v}_2 \cdot \vec{v}_2 - \vec{S}_1 \cdot \vec{S}_1 \vec{v}_1 \cdot \vec{v}_1 \vec{v}_2 \cdot \vec{v}_2 \right) \Big) m_2^2 C_{ES^2_1} \Big\}
\end{aligned}$$

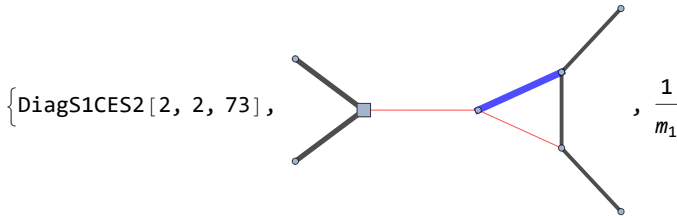

$$\begin{aligned}
& G^2 \left\{ \frac{1}{r^3} \left( -16 \hat{n} \cdot \vec{S}_1 \vec{S}_1 \cdot \vec{v}_1 \left( \hat{n} \cdot \vec{v}_2 \right)^2 + 32 \hat{n} \cdot \vec{v}_1 \vec{S}_1 \cdot \vec{S}_1 \left( \hat{n} \cdot \vec{v}_2 \right)^2 - 16 \hat{n} \cdot \vec{S}_1 \vec{S}_1 \cdot \vec{a}_1 \left( \hat{n} \cdot \vec{v}_2 \right)^2 - \right. \right. \\
& 16 \hat{n} \cdot \vec{S}_1 \vec{S}_1 \cdot \vec{v}_1 \left( \hat{n} \cdot \vec{v}_2 \right)^2 + 8 \vec{S}_1 \cdot \vec{v}_2 \vec{S}_1 \cdot \vec{v}_1 \hat{n} \cdot \vec{v}_2 + 8 \vec{S}_1 \cdot \vec{v}_1 \vec{S}_1 \cdot \vec{v}_2 \hat{n} \cdot \vec{v}_2 + 8 \vec{S}_1 \cdot \vec{a}_1 \vec{S}_1 \cdot \vec{v}_2 \hat{n} \cdot \vec{v}_2 - \\
& 16 \vec{S}_1 \cdot \vec{S}_1 \vec{v}_1 \cdot \vec{v}_2 \hat{n} \cdot \vec{v}_2 + 16 \hat{n} \cdot \vec{S}_1 \hat{n} \cdot \vec{S}_1 \vec{v}_2 \cdot \vec{v}_2 \hat{n} \cdot \vec{v}_2 + 4 \hat{n} \cdot \vec{S}_1 \vec{S}_1 \cdot \vec{v}_1 \vec{v}_2 \cdot \vec{v}_2 - 4 \hat{n} \cdot \vec{S}_1 \vec{S}_1 \cdot \vec{v}_2 \vec{v}_2 \cdot \vec{v}_2 - \\
& 8 \hat{n} \cdot \vec{v}_1 \vec{S}_1 \cdot \vec{S}_1 \vec{v}_2 \cdot \vec{v}_2 + 4 \hat{n} \cdot \vec{S}_1 \vec{S}_1 \cdot \vec{a}_1 \vec{v}_2 \cdot \vec{v}_2 + 4 \hat{n} \cdot \vec{S}_1 \vec{S}_1 \cdot \vec{v}_1 \vec{v}_2 \cdot \vec{v}_2 - 4 \hat{n} \cdot \vec{S}_1 \vec{S}_1 \cdot \vec{v}_2 \vec{v}_2 \cdot \vec{v}_2 \Big) + \\
& \frac{1}{r^4} \left( -16 \left( \vec{v}_2 \cdot \vec{v}_2 \right)^2 \left( \hat{n} \cdot \vec{S}_1 \right)^2 + 72 \left( \hat{n} \cdot \vec{v}_2 \right)^2 \vec{v}_1 \cdot \vec{v}_1 \left( \hat{n} \cdot \vec{S}_1 \right)^2 + 96 \left( \hat{n} \cdot \vec{v}_2 \right)^2 \vec{v}_2 \cdot \vec{v}_2 \left( \hat{n} \cdot \vec{S}_1 \right)^2 - \right. \\
& 48 \hat{n} \cdot \vec{v}_1 \hat{n} \cdot \vec{v}_2 \vec{v}_2 \cdot \vec{v}_2 \left( \hat{n} \cdot \vec{S}_1 \right)^2 - 12 \vec{v}_1 \cdot \vec{v}_1 \vec{v}_2 \cdot \vec{v}_2 \left( \hat{n} \cdot \vec{S}_1 \right)^2 + 8 \vec{v}_1 \cdot \vec{v}_2 \vec{v}_2 \cdot \vec{v}_2 \left( \hat{n} \cdot \vec{S}_1 \right)^2 - \\
& 48 \hat{n} \cdot \vec{v}_1 \left( \hat{n} \cdot \vec{v}_2 \right)^2 \vec{S}_1 \cdot \vec{v}_1 \hat{n} \cdot \vec{S}_1 - 48 \hat{n} \cdot \vec{v}_2 \vec{S}_1 \cdot \vec{v}_2 \vec{v}_1 \cdot \vec{v}_1 \hat{n} \cdot \vec{S}_1 + 16 \hat{n} \cdot \vec{v}_2 \vec{S}_1 \cdot \vec{v}_1 \vec{v}_1 \cdot \vec{v}_2 \hat{n} \cdot \vec{S}_1 + \\
& 8 \hat{n} \cdot \vec{v}_1 \vec{S}_1 \cdot \vec{v}_1 \vec{v}_2 \cdot \vec{v}_2 \hat{n} \cdot \vec{S}_1 + 16 \hat{n} \cdot \vec{v}_2 \vec{S}_1 \cdot \vec{v}_1 \vec{v}_2 \cdot \vec{v}_2 \hat{n} \cdot \vec{S}_1 + 16 \hat{n} \cdot \vec{v}_1 \vec{S}_1 \cdot \vec{v}_2 \vec{v}_2 \cdot \vec{v}_2 \hat{n} \cdot \vec{S}_1 - \\
& 64 \hat{n} \cdot \vec{v}_2 \vec{S}_1 \cdot \vec{v}_2 \vec{v}_2 \cdot \vec{v}_2 \hat{n} \cdot \vec{S}_1 + 8 \left( \hat{n} \cdot \vec{v}_2 \right)^2 \left( \vec{S}_1 \cdot \vec{v}_1 \right)^2 + 4 \vec{S}_1 \cdot \vec{S}_1 \left( \vec{v}_1 \cdot \vec{v}_2 \right)^2 + 48 \left( \hat{n} \cdot \vec{v}_1 \right)^2 \left( \hat{n} \cdot \vec{v}_2 \right)^2 \vec{S}_1 \cdot \vec{S}_1 + \\
& 16 \hat{n} \cdot \vec{v}_1 \hat{n} \cdot \vec{v}_2 \vec{S}_1 \cdot \vec{v}_1 \vec{S}_1 \cdot \vec{v}_2 + 6 \left( \vec{S}_1 \cdot \vec{v}_2 \right)^2 \vec{v}_1 \cdot \vec{v}_1 - 8 \left( \hat{n} \cdot \vec{v}_2 \right)^2 \vec{S}_1 \cdot \vec{S}_1 \vec{v}_1 \cdot \vec{v}_1 - 32 \hat{n} \cdot \vec{v}_1 \hat{n} \cdot \vec{v}_2 \vec{S}_1 \cdot \vec{S}_1 \vec{v}_1 \cdot \vec{v}_2 - \\
& 4 \vec{S}_1 \cdot \vec{v}_1 \vec{S}_1 \cdot \vec{v}_2 \vec{v}_1 \cdot \vec{v}_2 - 2 \left( \vec{S}_1 \cdot \vec{v}_1 \right)^2 \vec{v}_2 \cdot \vec{v}_2 + 8 \left( \vec{S}_1 \cdot \vec{v}_2 \right)^2 \vec{v}_2 \cdot \vec{v}_2 - 8 \left( \hat{n} \cdot \vec{v}_1 \right)^2 \vec{S}_1 \cdot \vec{S}_1 \vec{v}_2 \cdot \vec{v}_2 - \\
& \left. 4 \vec{S}_1 \cdot \vec{v}_1 \vec{S}_1 \cdot \vec{v}_2 \vec{v}_2 \cdot \vec{v}_2 + 2 \vec{S}_1 \cdot \vec{S}_1 \vec{v}_1 \cdot \vec{v}_1 \vec{v}_2 \cdot \vec{v}_2 \right) + \frac{2 \vec{v}_2 \cdot \vec{v}_2 \vec{S}_1^2 - 4 \left( \hat{n} \cdot \vec{v}_2 \right)^2 \vec{S}_1^2}{r^2} \Big\} m_2^2 C_{ES^2_1} \Big\}
\end{aligned}$$

$$\{\text{DiagS1CES2}[2, 2, 74],$$

[illegible]



$$\left. \frac{3}{2} \vec{S}_1 \cdot \vec{v}_1 \vec{S}_1 \cdot \vec{v}_2 \vec{v}_2 \cdot \vec{v}_2 + \frac{3}{2} \left( \hat{n} \cdot \vec{S}_1 \right)^2 \vec{v}_1 \cdot \vec{v}_1 \vec{v}_2 \cdot \vec{v}_2 + \frac{3}{2} \left( \hat{n} \cdot \vec{S}_1 \right)^2 \vec{v}_1 \cdot \vec{v}_2 \vec{v}_2 \cdot \vec{v}_2 \right) m_2 C_{ES^2_1} \Bigg\}$$

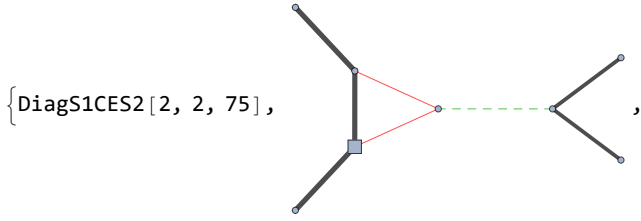

$$\begin{aligned} G^2 \Bigg( & \frac{1}{r^3} \left( -18 \hat{n} \cdot \vec{v}_2 \vec{v}_1 \cdot \vec{a}_1 \left( \hat{n} \cdot \vec{S}_1 \right)^2 - 3 \hat{n} \cdot \vec{v}_1 \hat{n} \cdot \vec{v}_2 \vec{S}_1 \cdot \vec{v}_1 \hat{n} \cdot \vec{S}_1 - 3 \hat{n} \cdot \vec{v}_1 \hat{n} \cdot \vec{v}_2 \vec{S}_1 \cdot \vec{a}_1 \hat{n} \cdot \vec{S}_1 + \hat{n} \cdot \vec{a}_1 \hat{n} \cdot \vec{v}_2 \vec{S}_1 \cdot \vec{v}_1 \hat{n} \cdot \vec{S}_1 - \right. \\ & \frac{1}{2} \vec{a}_1 \cdot \vec{v}_2 \vec{S}_1 \cdot \vec{v}_1 \hat{n} \cdot \vec{S}_1 + 9 \vec{S}_1 \cdot \vec{v}_2 \vec{v}_1 \cdot \vec{a}_1 \hat{n} \cdot \vec{S}_1 - 6 \hat{n} \cdot \vec{S}_1 \hat{n} \cdot \vec{v}_2 \vec{v}_1 \cdot \vec{v}_1 \hat{n} \cdot \vec{S}_1 + 3 \vec{S}_1 \cdot \vec{v}_2 \vec{v}_1 \cdot \vec{v}_1 \hat{n} \cdot \vec{S}_1 + \\ & \frac{3}{2} \vec{S}_1 \cdot \vec{v}_1 \vec{v}_1 \cdot \vec{v}_2 \hat{n} \cdot \vec{S}_1 + \frac{3}{2} \vec{S}_1 \cdot \vec{a}_1 \vec{v}_1 \cdot \vec{v}_2 \hat{n} \cdot \vec{S}_1 - \hat{n} \cdot \vec{S}_1 \hat{n} \cdot \vec{v}_2 \vec{v}_2 \cdot \vec{v}_2 \hat{n} \cdot \vec{S}_1 + \frac{1}{2} \vec{S}_1 \cdot \vec{v}_2 \vec{v}_2 \cdot \vec{v}_2 \hat{n} \cdot \vec{S}_1 + \\ & 6 \left( \hat{n} \cdot \vec{v}_1 \right)^2 \hat{n} \cdot \vec{v}_2 \vec{S}_1 \cdot \vec{S}_1 - 2 \hat{n} \cdot \vec{a}_1 \hat{n} \cdot \vec{v}_1 \hat{n} \cdot \vec{v}_2 \vec{S}_1 \cdot \vec{S}_1 + \hat{n} \cdot \vec{v}_1 \vec{a}_1 \cdot \vec{v}_2 \vec{S}_1 \cdot \vec{S}_1 - 3 \hat{n} \cdot \vec{S}_1 \hat{n} \cdot \vec{v}_1 \hat{n} \cdot \vec{v}_2 \vec{S}_1 \cdot \vec{v}_1 + \\ & 2 \hat{n} \cdot \vec{v}_2 \vec{S}_1 \cdot \vec{v}_1 \vec{S}_1 \cdot \vec{v}_1 + \frac{1}{2} \hat{n} \cdot \vec{v}_1 \vec{S}_1 \cdot \vec{v}_2 \vec{S}_1 \cdot \vec{v}_1 + \hat{n} \cdot \vec{v}_2 \vec{S}_1 \cdot \vec{a}_1 \vec{S}_1 \cdot \vec{v}_1 + \frac{1}{2} \hat{n} \cdot \vec{v}_1 \vec{S}_1 \cdot \vec{v}_1 \vec{S}_1 \cdot \vec{v}_2 + \frac{1}{2} \hat{n} \cdot \vec{v}_1 \vec{S}_1 \cdot \vec{a}_1 \\ & \vec{S}_1 \cdot \vec{v}_2 - \frac{1}{2} \hat{n} \cdot \vec{a}_1 \vec{S}_1 \cdot \vec{v}_1 \vec{S}_1 \cdot \vec{v}_2 + 3 \hat{n} \cdot \vec{v}_2 \vec{S}_1 \cdot \vec{S}_1 \vec{v}_1 \cdot \vec{a}_1 - 2 \hat{n} \cdot \vec{v}_2 \vec{S}_1 \cdot \vec{S}_1 \vec{v}_1 \cdot \vec{v}_1 + 3 \hat{n} \cdot \vec{S}_1 \vec{S}_1 \cdot \vec{v}_2 \vec{v}_1 \cdot \vec{v}_1 - \\ & 4 \hat{n} \cdot \vec{v}_1 \vec{S}_1 \cdot \vec{S}_1 \vec{v}_1 \cdot \vec{v}_2 + \hat{n} \cdot \vec{a}_1 \vec{S}_1 \cdot \vec{S}_1 \vec{v}_1 \cdot \vec{v}_2 + \frac{3}{2} \hat{n} \cdot \vec{S}_1 \vec{S}_1 \cdot \vec{v}_1 \vec{v}_1 \cdot \vec{v}_2 + \frac{1}{2} \hat{n} \cdot \vec{S}_1 \vec{S}_1 \cdot \vec{v}_2 \vec{v}_2 \cdot \vec{v}_2 \Bigg) + \frac{1}{r^4} \\ & \left( \frac{15}{2} \hat{n} \cdot \vec{v}_2 \vec{S}_1 \cdot \vec{S}_1 \left( \hat{n} \cdot \vec{v}_1 \right)^3 - \frac{15}{2} \hat{n} \cdot \vec{S}_1 \hat{n} \cdot \vec{v}_2 \vec{S}_1 \cdot \vec{v}_1 \left( \hat{n} \cdot \vec{v}_1 \right)^2 + \frac{3}{2} \vec{S}_1 \cdot \vec{v}_1 \vec{S}_1 \cdot \vec{v}_2 \left( \hat{n} \cdot \vec{v}_1 \right)^2 - \frac{11}{2} \vec{S}_1 \cdot \vec{S}_1 \right. \\ & \vec{v}_1 \cdot \vec{v}_2 \left( \hat{n} \cdot \vec{v}_1 \right)^2 + 2 \hat{n} \cdot \vec{v}_2 \left( \vec{S}_1 \cdot \vec{v}_1 \right)^2 \hat{n} \cdot \vec{v}_1 + \frac{45}{2} \left( \hat{n} \cdot \vec{S}_1 \right)^2 \hat{n} \cdot \vec{v}_2 \vec{v}_1 \cdot \vec{v}_1 \hat{n} \cdot \vec{v}_1 - 5 \hat{n} \cdot \vec{v}_2 \vec{S}_1 \cdot \vec{S}_1 \vec{v}_1 \cdot \vec{v}_1 \hat{n} \cdot \vec{v}_1 - \\ & 9 \hat{n} \cdot \vec{S}_1 \vec{S}_1 \cdot \vec{v}_2 \vec{v}_1 \cdot \vec{v}_1 \hat{n} \cdot \vec{v}_1 + 4 \hat{n} \cdot \vec{S}_1 \vec{S}_1 \cdot \vec{v}_1 \vec{v}_1 \cdot \vec{v}_2 \hat{n} \cdot \vec{v}_1 + \frac{15}{4} \left( \hat{n} \cdot \vec{S}_1 \right)^2 \hat{n} \cdot \vec{v}_2 \vec{v}_2 \cdot \vec{v}_2 \hat{n} \cdot \vec{v}_1 - \\ & \frac{1}{4} \hat{n} \cdot \vec{v}_2 \vec{S}_1 \cdot \vec{S}_1 \vec{v}_2 \cdot \vec{v}_2 \hat{n} \cdot \vec{v}_1 - \frac{3}{2} \hat{n} \cdot \vec{S}_1 \vec{S}_1 \cdot \vec{v}_2 \vec{v}_2 \cdot \vec{v}_2 \hat{n} \cdot \vec{v}_1 - \frac{15}{2} \hat{n} \cdot \vec{S}_1 \hat{n} \cdot \vec{v}_2 \vec{S}_1 \cdot \vec{v}_1 \vec{v}_1 \cdot \vec{v}_1 + \\ & \frac{5}{2} \vec{S}_1 \cdot \vec{v}_1 \vec{S}_1 \cdot \vec{v}_2 \vec{v}_1 \cdot \vec{v}_1 - \left( \vec{S}_1 \cdot \vec{v}_1 \right)^2 \vec{v}_1 \cdot \vec{v}_2 - \frac{15}{2} \left( \hat{n} \cdot \vec{S}_1 \right)^2 \vec{v}_1 \cdot \vec{v}_1 \vec{v}_1 \cdot \vec{v}_2 + 3 \vec{S}_1 \cdot \vec{S}_1 \vec{v}_1 \cdot \vec{v}_1 \vec{v}_1 \cdot \vec{v}_2 - \\ & \frac{3}{2} \hat{n} \cdot \vec{S}_1 \hat{n} \cdot \vec{v}_2 \vec{S}_1 \cdot \vec{v}_1 \vec{v}_2 \cdot \vec{v}_2 + \frac{1}{2} \vec{S}_1 \cdot \vec{v}_1 \vec{S}_1 \cdot \vec{v}_2 \vec{v}_2 \cdot \vec{v}_2 - \frac{5}{4} \left( \hat{n} \cdot \vec{S}_1 \right)^2 \vec{v}_1 \cdot \vec{v}_2 \vec{v}_2 \cdot \vec{v}_2 + \frac{1}{4} \vec{S}_1 \cdot \vec{S}_1 \vec{v}_1 \cdot \vec{v}_2 \vec{v}_2 \cdot \vec{v}_2 \Bigg) + \\ & \frac{1}{r^2} \left( -2 \hat{n} \cdot \vec{v}_1 \hat{n} \cdot \vec{v}_2 \vec{S}_1 \cdot \vec{S}_1 + 2 \vec{v}_1 \cdot \vec{v}_2 \vec{S}_1 \cdot \vec{S}_1 + 2 \hat{n} \cdot \vec{S}_1 \hat{n} \cdot \vec{v}_2 \vec{S}_1 \cdot \vec{a}_1 + 2 \hat{n} \cdot \vec{S}_1 \hat{n} \cdot \vec{v}_2 \vec{S}_1 \cdot \vec{v}_1 - 2 \vec{S}_1 \cdot \vec{v}_1 \vec{S}_1 \cdot \vec{v}_2 + \right. \\ & \hat{n} \cdot \vec{S}_1 \hat{n} \cdot \vec{v}_2 \vec{S}_1 \cdot \vec{v}_1 + \hat{n} \cdot \vec{S}_1 \hat{n} \cdot \vec{v}_2 \vec{S}_1 \cdot \vec{a}_1 - 4 \hat{n} \cdot \vec{a}_1 \hat{n} \cdot \vec{v}_2 \vec{S}_1 \cdot \vec{S}_1 + 4 \vec{a}_1 \cdot \vec{v}_2 \vec{S}_1 \cdot \vec{S}_1 - 2 \hat{n} \cdot \vec{v}_1 \hat{n} \cdot \vec{v}_2 \vec{S}_1 \cdot \vec{S}_1 + \\ & 2 \hat{n} \cdot \vec{S}_1 \hat{n} \cdot \vec{v}_2 \vec{S}_1 \cdot \vec{a}_1 - 2 \vec{S}_1 \cdot \vec{v}_2 \vec{S}_1 \cdot \vec{a}_1 + \hat{n} \cdot \vec{S}_1 \hat{n} \cdot \vec{v}_2 \vec{S}_1 \cdot \vec{v}_1 - \vec{S}_1 \cdot \vec{v}_2 \vec{S}_1 \cdot \vec{v}_1 - 2 \vec{S}_1 \cdot \vec{a}_1 \vec{S}_1 \cdot \vec{v}_2 - \vec{S}_1 \cdot \vec{v}_1 \vec{S}_1 \cdot \vec{v}_2 - \\ & \vec{S}_1 \cdot \vec{a}_1 \vec{S}_1 \cdot \vec{v}_2 + 2 \vec{S}_1 \cdot \vec{S}_1 \vec{v}_1 \cdot \vec{v}_2 + \hat{n} \cdot \vec{a}_1 \hat{n} \cdot \vec{v}_2 \vec{S}_1^2 - \vec{a}_1 \cdot \vec{v}_2 \vec{S}_1^2 - 2 \hat{n} \cdot \vec{v}_1 \hat{n} \cdot \vec{v}_2 \vec{S}_1^2 + 2 \vec{v}_1 \cdot \vec{v}_2 \vec{S}_1^2 \Bigg) + \frac{2 \hat{n} \cdot \vec{v}_2 \vec{S}_1^3}{r} \Bigg) m_2 C_{ES^2_1} \Bigg\} \end{aligned}$$

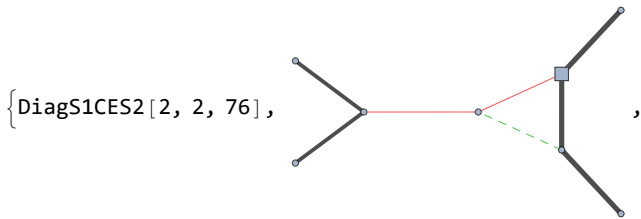

$\{\text{DiagS1CES2}[2, 2, 77],$ 
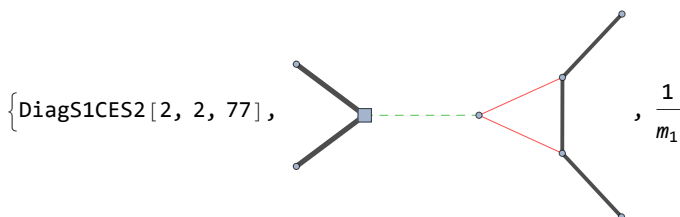
 $, \frac{1}{m_1}$

$$\begin{aligned}
G^2 \left( -\frac{12 \hat{n} \cdot \vec{S}_1 \hat{n} \cdot \vec{S}_1 \vec{v}_2 \cdot \vec{a}_2}{r^2} + \frac{1}{r^3} \left( -2 \hat{n} \cdot \vec{v}_2 \vec{v}_1 \cdot \vec{a}_1 (\hat{n} \cdot \vec{S}_1)^2 + 24 \hat{n} \cdot \vec{v}_1 \vec{v}_2 \cdot \vec{a}_2 (\hat{n} \cdot \vec{S}_1)^2 + 2 \hat{n} \cdot \vec{v}_1 \hat{n} \cdot \vec{v}_2 \vec{S}_1 \cdot \vec{v}_1 \hat{n} \cdot \vec{S}_1 + \right. \right. \\
2 \hat{n} \cdot \vec{v}_1 \hat{n} \cdot \vec{v}_2 \vec{S}_1 \cdot \vec{a}_1 \hat{n} \cdot \vec{S}_1 + 2 \hat{n} \cdot \vec{a}_1 \hat{n} \cdot \vec{v}_2 \vec{S}_1 \cdot \vec{v}_1 \hat{n} \cdot \vec{S}_1 - \frac{3}{4} \vec{a}_1 \cdot \vec{v}_2 \vec{S}_1 \cdot \vec{v}_1 \hat{n} \cdot \vec{S}_1 + \frac{3}{2} \vec{S}_1 \cdot \vec{v}_2 \vec{v}_1 \cdot \vec{a}_1 \hat{n} \cdot \vec{S}_1 - \\
2 \hat{n} \cdot \vec{S}_1 \hat{n} \cdot \vec{v}_2 \vec{v}_1 \cdot \vec{v}_1 \hat{n} \cdot \vec{S}_1 + \frac{3}{4} \vec{S}_1 \cdot \vec{v}_2 \vec{v}_1 \cdot \vec{v}_1 \hat{n} \cdot \vec{S}_1 - \frac{3}{4} \vec{S}_1 \cdot \vec{v}_1 \vec{v}_1 \cdot \vec{v}_2 \hat{n} \cdot \vec{S}_1 - \frac{3}{4} \vec{S}_1 \cdot \vec{a}_1 \vec{v}_1 \cdot \vec{v}_2 \hat{n} \cdot \vec{S}_1 - \\
12 \vec{S}_1 \cdot \vec{v}_1 \vec{v}_2 \cdot \vec{a}_2 \hat{n} \cdot \vec{S}_1 - 12 \hat{n} \cdot \vec{S}_1 \hat{n} \cdot \vec{v}_2 \vec{v}_2 \cdot \vec{v}_2 \hat{n} \cdot \vec{S}_1 + \frac{9}{2} \vec{S}_1 \cdot \vec{v}_2 \vec{v}_2 \cdot \vec{v}_2 \hat{n} \cdot \vec{S}_1 - 4 (\hat{n} \cdot \vec{v}_1)^2 \hat{n} \cdot \vec{v}_2 \vec{S}_1 \cdot \vec{S}_1 - \\
4 \hat{n} \cdot \vec{a}_1 \hat{n} \cdot \vec{v}_1 \hat{n} \cdot \vec{v}_2 \vec{S}_1 \cdot \vec{S}_1 + \frac{3}{2} \hat{n} \cdot \vec{v}_1 \vec{a}_1 \cdot \vec{v}_2 \vec{S}_1 \cdot \vec{S}_1 + 2 \hat{n} \cdot \vec{S}_1 \hat{n} \cdot \vec{v}_1 \hat{n} \cdot \vec{v}_2 \vec{S}_1 \cdot \vec{v}_1 - \hat{n} \cdot \vec{v}_2 \vec{S}_1 \cdot \vec{v}_1 \vec{S}_1 \cdot \vec{v}_1 - \\
\frac{3}{4} \hat{n} \cdot \vec{v}_1 \vec{S}_1 \cdot \vec{v}_2 \vec{S}_1 \cdot \vec{v}_1 - \hat{n} \cdot \vec{v}_2 \vec{S}_1 \cdot \vec{a}_1 \vec{S}_1 \cdot \vec{v}_1 - \frac{3}{4} \hat{n} \cdot \vec{v}_1 \vec{S}_1 \cdot \vec{v}_1 \vec{S}_1 \cdot \vec{v}_2 - \frac{3}{4} \hat{n} \cdot \vec{v}_1 \vec{S}_1 \cdot \vec{a}_1 \vec{S}_1 \cdot \vec{v}_2 - \frac{3}{4} \hat{n} \cdot \vec{a}_1 \vec{S}_1 \cdot \vec{v}_1 \\
\vec{S}_1 \cdot \vec{v}_2 + \frac{1}{2} \hat{n} \cdot \vec{v}_2 \vec{S}_1 \cdot \vec{S}_1 \vec{v}_1 \cdot \vec{a}_1 + \frac{1}{2} \hat{n} \cdot \vec{v}_2 \vec{S}_1 \cdot \vec{S}_1 \vec{v}_1 \cdot \vec{v}_1 + \frac{3}{4} \hat{n} \cdot \vec{S}_1 \vec{S}_1 \cdot \vec{v}_2 \vec{v}_1 \cdot \vec{v}_1 + 3 \hat{n} \cdot \vec{v}_1 \vec{S}_1 \cdot \vec{S}_1 \vec{v}_1 \cdot \vec{v}_2 + \\
\left. \frac{3}{2} \hat{n} \cdot \vec{a}_1 \vec{S}_1 \cdot \vec{S}_1 \vec{v}_1 \cdot \vec{v}_2 - \frac{3}{4} \hat{n} \cdot \vec{S}_1 \vec{S}_1 \cdot \vec{v}_1 \vec{v}_1 \cdot \vec{v}_2 - 3 \hat{n} \cdot \vec{v}_2 \vec{S}_1 \cdot \vec{S}_1 \vec{v}_2 \cdot \vec{v}_2 + \frac{9}{2} \hat{n} \cdot \vec{S}_1 \vec{S}_1 \cdot \vec{v}_2 \vec{v}_2 \cdot \vec{v}_2 \right) + \\
\frac{1}{r^4} \left( 12 \hat{n} \cdot \vec{v}_2 \vec{S}_1 \cdot \vec{S}_1 (\hat{n} \cdot \vec{v}_1)^3 - 12 \hat{n} \cdot \vec{S}_1 \hat{n} \cdot \vec{v}_2 \vec{S}_1 \cdot \vec{v}_1 (\hat{n} \cdot \vec{v}_1)^2 + 2 \vec{S}_1 \cdot \vec{v}_1 \vec{S}_1 \cdot \vec{v}_2 (\hat{n} \cdot \vec{v}_1)^2 - \right. \\
8 \vec{S}_1 \cdot \vec{S}_1 \vec{v}_1 \cdot \vec{v}_2 (\hat{n} \cdot \vec{v}_1)^2 + 4 \hat{n} \cdot \vec{v}_2 (\vec{S}_1 \cdot \vec{v}_1)^2 \hat{n} \cdot \vec{v}_1 + 6 (\hat{n} \cdot \vec{S}_1)^2 \hat{n} \cdot \vec{v}_2 \vec{v}_1 \cdot \vec{v}_1 \hat{n} \cdot \vec{v}_1 - \\
6 \hat{n} \cdot \vec{v}_2 \vec{S}_1 \cdot \vec{S}_1 \vec{v}_1 \cdot \vec{v}_1 \hat{n} \cdot \vec{v}_1 - 2 \hat{n} \cdot \vec{S}_1 \vec{S}_1 \cdot \vec{v}_2 \vec{v}_1 \cdot \vec{v}_1 \hat{n} \cdot \vec{v}_1 + 6 \hat{n} \cdot \vec{S}_1 \vec{S}_1 \cdot \vec{v}_1 \vec{v}_1 \cdot \vec{v}_2 \hat{n} \cdot \vec{v}_1 + \\
36 (\hat{n} \cdot \vec{S}_1)^2 \hat{n} \cdot \vec{v}_2 \vec{v}_2 \cdot \vec{v}_2 \hat{n} \cdot \vec{v}_1 - 12 \hat{n} \cdot \vec{S}_1 \vec{S}_1 \cdot \vec{v}_2 \vec{v}_2 \cdot \vec{v}_2 \hat{n} \cdot \vec{v}_1 - \frac{3}{2} (\vec{S}_1 \cdot \vec{v}_1)^2 \vec{v}_1 \cdot \vec{v}_2 - \\
2 (\hat{n} \cdot \vec{S}_1)^2 \vec{v}_1 \cdot \vec{v}_1 \vec{v}_1 \cdot \vec{v}_2 + \frac{5}{2} \vec{S}_1 \cdot \vec{S}_1 \vec{v}_1 \cdot \vec{v}_1 \vec{v}_1 \cdot \vec{v}_2 - 12 \hat{n} \cdot \vec{S}_1 \hat{n} \cdot \vec{v}_2 \vec{S}_1 \cdot \vec{v}_1 \vec{v}_2 \cdot \vec{v}_2 + \\
\left. 3 \vec{S}_1 \cdot \vec{v}_1 \vec{S}_1 \cdot \vec{v}_2 \vec{v}_2 \cdot \vec{v}_2 - 12 (\hat{n} \cdot \vec{S}_1)^2 \vec{v}_1 \cdot \vec{v}_2 \vec{v}_2 \cdot \vec{v}_2 + 3 \vec{S}_1 \cdot \vec{S}_1 \vec{v}_1 \cdot \vec{v}_2 \vec{v}_2 \cdot \vec{v}_2 \right) \Bigg\} m_2^2 C_{ES^2 1} \Bigg\}
\end{aligned}$$

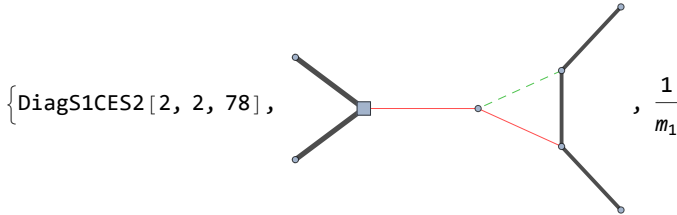

$$\begin{aligned}
G^2 \left( \frac{1}{r^3} \left( 24 \hat{n} \cdot \vec{v}_2 \vec{v}_1 \cdot \vec{a}_1 (\hat{n} \cdot \vec{S}_1)^2 - 48 \hat{n} \cdot \vec{v}_2 \vec{v}_2 \cdot \vec{a}_2 (\hat{n} \cdot \vec{S}_1)^2 + 16 (\hat{n} \cdot \vec{v}_2)^2 \vec{S}_1 \cdot \vec{v}_1 \hat{n} \cdot \vec{S}_1 + \right. \right. \\
8 \hat{n} \cdot \vec{v}_1 \hat{n} \cdot \vec{v}_2 \vec{S}_1 \cdot \vec{v}_1 \hat{n} \cdot \vec{S}_1 + 16 (\hat{n} \cdot \vec{v}_2)^2 \vec{S}_1 \cdot \vec{a}_1 \hat{n} \cdot \vec{S}_1 + 8 \hat{n} \cdot \vec{v}_1 \hat{n} \cdot \vec{v}_2 \vec{S}_1 \cdot \vec{a}_1 \hat{n} \cdot \vec{S}_1 - \\
8 \hat{n} \cdot \vec{a}_1 \hat{n} \cdot \vec{v}_2 \vec{S}_1 \cdot \vec{v}_1 \hat{n} \cdot \vec{S}_1 + 2 \vec{a}_1 \cdot \vec{v}_2 \vec{S}_1 \cdot \vec{v}_1 \hat{n} \cdot \vec{S}_1 - 12 \vec{S}_1 \cdot \vec{v}_2 \vec{v}_1 \cdot \vec{a}_1 \hat{n} \cdot \vec{S}_1 + 24 \hat{n} \cdot \vec{S}_1 \hat{n} \cdot \vec{v}_2 \vec{v}_1 \cdot \vec{v}_1 \hat{n} \cdot \vec{S}_1 - \\
6 \vec{S}_1 \cdot \vec{v}_2 \vec{v}_1 \cdot \vec{v}_1 \hat{n} \cdot \vec{S}_1 - 2 \vec{S}_1 \cdot \vec{v}_1 \vec{v}_1 \cdot \vec{v}_2 \hat{n} \cdot \vec{S}_1 - 2 \vec{S}_1 \cdot \vec{a}_1 \vec{v}_1 \cdot \vec{v}_2 \hat{n} \cdot \vec{S}_1 + 24 \vec{S}_1 \cdot \vec{v}_2 \vec{v}_2 \cdot \vec{a}_2 \hat{n} \cdot \vec{S}_1 + \\
32 \hat{n} \cdot \vec{S}_1 \hat{n} \cdot \vec{v}_2 \vec{v}_2 \cdot \vec{v}_2 \hat{n} \cdot \vec{S}_1 - 4 \vec{S}_1 \cdot \vec{v}_1 \vec{v}_2 \cdot \vec{v}_2 \hat{n} \cdot \vec{S}_1 - 8 \vec{S}_1 \cdot \vec{v}_2 \vec{v}_2 \cdot \vec{v}_2 \hat{n} \cdot \vec{S}_1 - 4 \vec{S}_1 \cdot \vec{a}_1 \vec{v}_2 \cdot \vec{v}_2 \hat{n} \cdot \vec{S}_1 - \\
32 \hat{n} \cdot \vec{v}_1 (\hat{n} \cdot \vec{v}_2)^2 \vec{S}_1 \cdot \vec{S}_1 - 16 (\hat{n} \cdot \vec{v}_1)^2 \hat{n} \cdot \vec{v}_2 \vec{S}_1 \cdot \vec{S}_1 + 16 \hat{n} \cdot \vec{a}_1 \hat{n} \cdot \vec{v}_1 \hat{n} \cdot \vec{v}_2 \vec{S}_1 \cdot \vec{S}_1 - 4 \hat{n} \cdot \vec{v}_1 \vec{a}_1 \cdot \vec{v}_2 \vec{S}_1 \cdot \vec{S}_1 + \\
16 \hat{n} \cdot \vec{S}_1 (\hat{n} \cdot \vec{v}_2)^2 \vec{S}_1 \cdot \vec{v}_1 + 8 \hat{n} \cdot \vec{S}_1 \hat{n} \cdot \vec{v}_1 \hat{n} \cdot \vec{v}_2 \vec{S}_1 \cdot \vec{v}_1 - 4 \hat{n} \cdot \vec{v}_2 \vec{S}_1 \cdot \vec{v}_1 \vec{S}_1 \cdot \vec{v}_1 - 2 \hat{n} \cdot \vec{v}_1 \vec{S}_1 \cdot \vec{v}_2 \vec{S}_1 \cdot \vec{v}_1 - \\
8 \hat{n} \cdot \vec{v}_2 \vec{S}_1 \cdot \vec{v}_2 \vec{S}_1 \cdot \vec{v}_1 - 2 \hat{n} \cdot \vec{v}_1 \vec{S}_1 \cdot \vec{v}_1 \vec{S}_1 \cdot \vec{v}_2 - 8 \hat{n} \cdot \vec{v}_2 \vec{S}_1 \cdot \vec{v}_1 \vec{S}_1 \cdot \vec{v}_2 - 2 \hat{n} \cdot \vec{v}_1 \vec{S}_1 \cdot \vec{a}_1 \vec{S}_1 \cdot \vec{v}_2 - \\
8 \hat{n} \cdot \vec{v}_2 \vec{S}_1 \cdot \vec{a}_1 \vec{S}_1 \cdot \vec{v}_2 + 2 \hat{n} \cdot \vec{a}_1 \vec{S}_1 \cdot \vec{v}_1 \vec{S}_1 \cdot \vec{v}_2 - 4 \hat{n} \cdot \vec{v}_2 \vec{S}_1 \cdot \vec{S}_1 \vec{v}_1 \cdot \vec{a}_1 + 4 \hat{n} \cdot \vec{v}_2 \vec{S}_1 \cdot \vec{S}_1 \vec{v}_1 \cdot \vec{v}_1 - \\
\left. \left. \right) \right\} m_2^2 C_{ES^2 1} \Bigg\}
\end{aligned}$$

$$\begin{aligned}
& 6 \hat{n} \cdot \vec{S}_1 \vec{S}_1 \cdot \vec{v}_2 \vec{v}_1 \cdot \vec{v}_1 + 8 \hat{n} \cdot \vec{v}_1 \vec{S}_1 \cdot \vec{S}_1 \vec{v}_1 \cdot \vec{v}_2 + 16 \hat{n} \cdot \vec{v}_2 \vec{S}_1 \cdot \vec{S}_1 \vec{v}_1 \cdot \vec{v}_2 - 4 \hat{n} \cdot \vec{a}_1 \vec{S}_1 \cdot \vec{S}_1 \vec{v}_1 \cdot \vec{v}_2 - \\
& 2 \hat{n} \cdot \vec{S}_1 \vec{S}_1 \cdot \vec{v}_1 \vec{v}_1 \cdot \vec{v}_2 + 8 \hat{n} \cdot \vec{v}_1 \vec{S}_1 \cdot \vec{S}_1 \vec{v}_2 \cdot \vec{v}_2 - 4 \hat{n} \cdot \vec{S}_1 \vec{S}_1 \cdot \vec{v}_1 \vec{v}_2 \cdot \vec{v}_2 - 8 \hat{n} \cdot \vec{S}_1 \vec{S}_1 \cdot \vec{v}_2 \vec{v}_2 \cdot \vec{v}_2 \Big) + \\
& \frac{1}{\rho^4} \Big( -48 \hat{n} \cdot \vec{v}_2 \vec{S}_1 \cdot \vec{S}_1 (\hat{n} \cdot \vec{v}_1)^3 - 48 (\hat{n} \cdot \vec{v}_2)^2 \vec{S}_1 \cdot \vec{S}_1 (\hat{n} \cdot \vec{v}_1)^2 + 48 \hat{n} \cdot \vec{S}_1 \hat{n} \cdot \vec{v}_2 \vec{S}_1 \cdot \vec{v}_1 (\hat{n} \cdot \vec{v}_1)^2 - \\
& 8 \vec{S}_1 \cdot \vec{v}_1 \vec{S}_1 \cdot \vec{v}_2 (\hat{n} \cdot \vec{v}_1)^2 + 24 \vec{S}_1 \cdot \vec{S}_1 \vec{v}_1 \cdot \vec{v}_2 (\hat{n} \cdot \vec{v}_1)^2 + 8 \vec{S}_1 \cdot \vec{S}_1 \vec{v}_2 \cdot \vec{v}_2 (\hat{n} \cdot \vec{v}_1)^2 - 16 \hat{n} \cdot \vec{v}_2 (\vec{S}_1 \cdot \vec{v}_1)^2 \hat{n} \cdot \vec{v}_1 + \\
& 48 \hat{n} \cdot \vec{S}_1 (\hat{n} \cdot \vec{v}_2)^2 \vec{S}_1 \cdot \vec{v}_1 \hat{n} \cdot \vec{v}_1 - 16 \hat{n} \cdot \vec{v}_2 \vec{S}_1 \cdot \vec{v}_1 \vec{S}_1 \cdot \vec{v}_2 \hat{n} \cdot \vec{v}_1 - 72 (\hat{n} \cdot \vec{S}_1)^2 \hat{n} \cdot \vec{v}_2 \vec{v}_1 \cdot \vec{v}_1 \hat{n} \cdot \vec{v}_1 + \\
& 24 \hat{n} \cdot \vec{v}_2 \vec{S}_1 \cdot \vec{S}_1 \vec{v}_1 \cdot \vec{v}_1 \hat{n} \cdot \vec{v}_1 + 24 \hat{n} \cdot \vec{S}_1 \vec{S}_1 \cdot \vec{v}_2 \vec{v}_1 \cdot \vec{v}_1 \hat{n} \cdot \vec{v}_1 + 32 \hat{n} \cdot \vec{v}_2 \vec{S}_1 \cdot \vec{S}_1 \vec{v}_1 \cdot \vec{v}_2 \hat{n} \cdot \vec{v}_1 - \\
& 16 \hat{n} \cdot \vec{S}_1 \vec{S}_1 \cdot \vec{v}_1 \vec{v}_1 \cdot \vec{v}_2 \hat{n} \cdot \vec{v}_1 - 96 (\hat{n} \cdot \vec{S}_1)^2 \hat{n} \cdot \vec{v}_2 \vec{v}_2 \cdot \vec{v}_2 \hat{n} \cdot \vec{v}_1 - 8 \hat{n} \cdot \vec{S}_1 \vec{S}_1 \cdot \vec{v}_1 \vec{v}_2 \cdot \vec{v}_2 \hat{n} \cdot \vec{v}_1 + \\
& 32 \hat{n} \cdot \vec{S}_1 \vec{S}_1 \cdot \vec{v}_2 \vec{v}_2 \cdot \vec{v}_2 \hat{n} \cdot \vec{v}_1 - 8 (\hat{n} \cdot \vec{v}_2)^2 (\vec{S}_1 \cdot \vec{v}_1)^2 - 4 \vec{S}_1 \cdot \vec{S}_1 (\vec{v}_1 \cdot \vec{v}_2)^2 + 16 (\hat{n} \cdot \vec{S}_1)^2 (\vec{v}_2 \cdot \vec{v}_2)^2 - \\
& 72 (\hat{n} \cdot \vec{S}_1)^2 (\hat{n} \cdot \vec{v}_2)^2 \vec{v}_1 \cdot \vec{v}_1 - 6 (\vec{S}_1 \cdot \vec{v}_2)^2 \vec{v}_1 \cdot \vec{v}_1 + 8 (\hat{n} \cdot \vec{v}_2)^2 \vec{S}_1 \cdot \vec{S}_1 \vec{v}_1 \cdot \vec{v}_1 + 16 \hat{n} \cdot \vec{S}_1 \hat{n} \cdot \vec{v}_2 \vec{S}_1 \cdot \vec{v}_1 \vec{v}_1 \cdot \vec{v}_1 + \\
& 48 \hat{n} \cdot \vec{S}_1 \hat{n} \cdot \vec{v}_2 \vec{S}_1 \cdot \vec{v}_2 \vec{v}_1 \cdot \vec{v}_1 - 4 \vec{S}_1 \cdot \vec{v}_1 \vec{S}_1 \cdot \vec{v}_2 \vec{v}_1 \cdot \vec{v}_1 + 4 (\vec{S}_1 \cdot \vec{v}_1)^2 \vec{v}_1 \cdot \vec{v}_2 - 16 \hat{n} \cdot \vec{S}_1 \hat{n} \cdot \vec{v}_2 \vec{S}_1 \cdot \vec{v}_1 \vec{v}_1 \cdot \vec{v}_2 + \\
& 4 \vec{S}_1 \cdot \vec{v}_1 \vec{S}_1 \cdot \vec{v}_2 \vec{v}_1 \cdot \vec{v}_2 + 12 (\hat{n} \cdot \vec{S}_1)^2 \vec{v}_1 \cdot \vec{v}_1 \vec{v}_1 \cdot \vec{v}_2 - 6 \vec{S}_1 \cdot \vec{S}_1 \vec{v}_1 \cdot \vec{v}_1 \vec{v}_1 \cdot \vec{v}_2 - 96 (\hat{n} \cdot \vec{S}_1)^2 (\hat{n} \cdot \vec{v}_2)^2 \vec{v}_2 \cdot \vec{v}_2 + \\
& 2 (\vec{S}_1 \cdot \vec{v}_1)^2 \vec{v}_2 \cdot \vec{v}_2 - 8 (\vec{S}_1 \cdot \vec{v}_2)^2 \vec{v}_2 \cdot \vec{v}_2 + 32 \hat{n} \cdot \vec{S}_1 \hat{n} \cdot \vec{v}_2 \vec{S}_1 \cdot \vec{v}_1 \vec{v}_2 \cdot \vec{v}_2 + 64 \hat{n} \cdot \vec{S}_1 \hat{n} \cdot \vec{v}_2 \vec{S}_1 \cdot \vec{v}_2 \vec{v}_2 \cdot \vec{v}_2 - \\
& 8 \vec{S}_1 \cdot \vec{v}_1 \vec{S}_1 \cdot \vec{v}_2 \vec{v}_2 \cdot \vec{v}_2 + 12 (\hat{n} \cdot \vec{S}_1)^2 \vec{v}_1 \cdot \vec{v}_1 \vec{v}_2 \cdot \vec{v}_2 - 2 \vec{S}_1 \cdot \vec{S}_1 \vec{v}_1 \cdot \vec{v}_1 \vec{v}_2 \cdot \vec{v}_2 + 16 (\hat{n} \cdot \vec{S}_1)^2 \vec{v}_1 \cdot \vec{v}_2 \vec{v}_2 \cdot \vec{v}_2 \Big) + \frac{1}{\rho^2} \\
& \Big( 4 \vec{S}_1^2 (\hat{n} \cdot \vec{v}_2)^2 + 8 \hat{n} \cdot \vec{v}_1 \vec{S}_1 \cdot \vec{S}_1 \hat{n} \cdot \vec{v}_2 - 8 \hat{n} \cdot \vec{S}_1 \vec{S}_1 \cdot \vec{a}_1 \hat{n} \cdot \vec{v}_2 - 8 \hat{n} \cdot \vec{S}_1 \vec{S}_1 \cdot \vec{v}_1 \hat{n} \cdot \vec{v}_2 - 4 \hat{n} \cdot \vec{S}_1 \vec{S}_1 \cdot \vec{v}_1 \hat{n} \cdot \vec{v}_2 - \\
& 4 \hat{n} \cdot \vec{S}_1 \vec{S}_1 \cdot \vec{a}_1 \hat{n} \cdot \vec{v}_2 + 16 \hat{n} \cdot \vec{a}_1 \vec{S}_1 \cdot \vec{S}_1 \hat{n} \cdot \vec{v}_2 + 8 \hat{n} \cdot \vec{v}_1 \vec{S}_1 \cdot \vec{S}_1 \hat{n} \cdot \vec{v}_2 - 8 \hat{n} \cdot \vec{S}_1 \vec{S}_1 \cdot \vec{a}_1 \hat{n} \cdot \vec{v}_2 - \\
& 4 \hat{n} \cdot \vec{S}_1 \vec{S}_1 \cdot \vec{v}_1 \hat{n} \cdot \vec{v}_2 - 4 \hat{n} \cdot \vec{a}_1 \vec{S}_1^2 \hat{n} \cdot \vec{v}_2 + 4 \hat{n} \cdot \vec{v}_1 \vec{S}_1^2 \hat{n} \cdot \vec{v}_2 + 4 \vec{S}_1 \cdot \vec{v}_1 \vec{S}_1 \cdot \vec{v}_2 - 8 \vec{a}_1 \cdot \vec{v}_2 \vec{S}_1 \cdot \vec{S}_1 + \\
& 4 \vec{S}_1 \cdot \vec{v}_2 \vec{S}_1 \cdot \vec{a}_1 + 2 \vec{S}_1 \cdot \vec{v}_2 \vec{S}_1 \cdot \vec{v}_1 + 4 \vec{S}_1 \cdot \vec{a}_1 \vec{S}_1 \cdot \vec{v}_2 + 2 \vec{S}_1 \cdot \vec{v}_1 \vec{S}_1 \cdot \vec{v}_2 + 2 \vec{S}_1 \cdot \vec{a}_1 \vec{S}_1 \cdot \vec{v}_2 - \\
& 4 \vec{S}_1 \cdot \vec{S}_1 \vec{v}_1 \cdot \vec{v}_2 - 4 \vec{S}_1 \cdot \vec{S}_1 \vec{v}_1 \cdot \vec{v}_2 + 2 \vec{a}_1 \cdot \vec{v}_2 \vec{S}_1^2 - 2 \vec{v}_1 \cdot \vec{v}_2 \vec{S}_1^2 - 2 \vec{v}_2 \cdot \vec{v}_2 \vec{S}_1^2 \Big) - \frac{2 \hat{n} \cdot \vec{v}_2 \vec{S}_1^2}{r} \Big) m_2^2 C_{ES^1} \Big\}
\end{aligned}$$

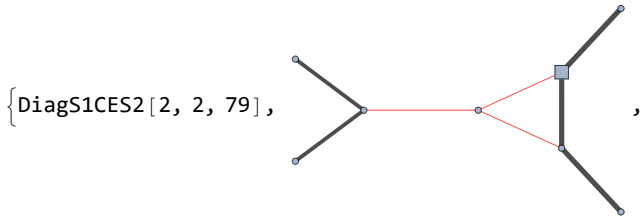

$$\begin{aligned}
& G^2 \left( \frac{1}{\rho^3} \left( -2 \vec{S}_1 \cdot \vec{S}_1 (\hat{n} \cdot \vec{v}_1)^3 + \hat{n} \cdot \vec{S}_1 \vec{S}_1 \cdot \vec{v}_1 (\hat{n} \cdot \vec{v}_1)^2 + 20 \hat{n} \cdot \vec{v}_2 \vec{S}_1 \cdot \vec{S}_1 (\hat{n} \cdot \vec{v}_1)^2 + \right. \right. \\
& \hat{n} \cdot \vec{S}_1 \vec{S}_1 \cdot \vec{a}_1 (\hat{n} \cdot \vec{v}_1)^2 + 2 \hat{n} \cdot \vec{a}_1 \vec{S}_1 \cdot \vec{S}_1 (\hat{n} \cdot \vec{v}_1)^2 + \hat{n} \cdot \vec{S}_1 \vec{S}_1 \cdot \vec{v}_1 (\hat{n} \cdot \vec{v}_1)^2 - 10 \hat{n} \cdot \vec{S}_1 \hat{n} \cdot \vec{v}_2 \vec{S}_1 \cdot \vec{v}_1 \hat{n} \cdot \vec{v}_1 - \\
& 10 \hat{n} \cdot \vec{S}_1 \hat{n} \cdot \vec{v}_2 \vec{S}_1 \cdot \vec{a}_1 \hat{n} \cdot \vec{v}_1 - 12 \hat{n} \cdot \vec{a}_1 \hat{n} \cdot \vec{v}_2 \vec{S}_1 \cdot \vec{S}_1 \hat{n} \cdot \vec{v}_1 + 3 \vec{a}_1 \cdot \vec{v}_2 \vec{S}_1 \cdot \vec{S}_1 \hat{n} \cdot \vec{v}_1 - \\
& \hat{n} \cdot \vec{a}_1 \hat{n} \cdot \vec{S}_1 \vec{S}_1 \cdot \vec{v}_1 \hat{n} \cdot \vec{v}_1 - 10 \hat{n} \cdot \vec{S}_1 \hat{n} \cdot \vec{v}_2 \vec{S}_1 \cdot \vec{v}_1 \hat{n} \cdot \vec{v}_1 - \vec{S}_1 \cdot \vec{v}_1 \vec{S}_1 \cdot \vec{v}_1 \hat{n} \cdot \vec{v}_1 + \frac{5}{2} \vec{S}_1 \cdot \vec{v}_2 \vec{S}_1 \cdot \vec{v}_1 \hat{n} \cdot \vec{v}_1 - \\
& \frac{1}{2} \vec{S}_1 \cdot \vec{a}_1 \vec{S}_1 \cdot \vec{v}_1 \hat{n} \cdot \vec{v}_1 + \frac{5}{2} \vec{S}_1 \cdot \vec{v}_1 \vec{S}_1 \cdot \vec{v}_2 \hat{n} \cdot \vec{v}_1 + \frac{5}{2} \vec{S}_1 \cdot \vec{a}_1 \vec{S}_1 \cdot \vec{v}_2 \hat{n} \cdot \vec{v}_1 + 18 (\hat{n} \cdot \vec{S}_1)^2 \vec{v}_1 \cdot \vec{a}_1 \hat{n} \cdot \vec{v}_1 - \\
& 4 \vec{S}_1 \cdot \vec{S}_1 \vec{v}_1 \cdot \vec{a}_1 \hat{n} \cdot \vec{v}_1 + 6 \hat{n} \cdot \vec{S}_1 \hat{n} \cdot \vec{S}_1 \vec{v}_1 \cdot \vec{v}_1 \hat{n} \cdot \vec{v}_1 + 2 \vec{S}_1 \cdot \vec{S}_1 \vec{v}_1 \cdot \vec{v}_1 \hat{n} \cdot \vec{v}_1 - 10 \vec{S}_1 \cdot \vec{S}_1 \vec{v}_1 \cdot \vec{v}_2 \hat{n} \cdot \vec{v}_1 + \\
& 18 (\hat{n} \cdot \vec{S}_1)^2 \vec{v}_2 \cdot \vec{a}_2 \hat{n} \cdot \vec{v}_1 - 3 \vec{S}_1 \cdot \vec{S}_1 \vec{v}_2 \cdot \vec{a}_2 \hat{n} \cdot \vec{v}_1 + 3 \hat{n} \cdot \vec{S}_1 \hat{n} \cdot \vec{S}_1 \vec{v}_2 \cdot \vec{v}_2 \hat{n} \cdot \vec{v}_1 + \frac{1}{2} \hat{n} \cdot \vec{a}_1 (\vec{S}_1 \cdot \vec{v}_1)^2 + \\
& \left. \left. 6 \hat{n} \cdot \vec{a}_1 \hat{n} \cdot \vec{S}_1 \hat{n} \cdot \vec{v}_2 \vec{S}_1 \cdot \vec{v}_1 + 6 \hat{n} \cdot \vec{v}_2 \vec{S}_1 \cdot \vec{v}_1 \vec{S}_1 \cdot \vec{v}_1 - \frac{3}{2} \hat{n} \cdot \vec{S}_1 \vec{a}_1 \cdot \vec{v}_2 \vec{S}_1 \cdot \vec{v}_1 + 2 \hat{n} \cdot \vec{v}_2 \vec{S}_1 \cdot \vec{a}_1 \vec{S}_1 \cdot \vec{v}_1 - \right. \right.
\end{aligned}$$



$$\{\text{DiagS1CES2}[2, 2, 80],$$

[illegible]

$$4 \vec{S}_1 \cdot \vec{S}_1 \vec{v}_1 \cdot \vec{v}_2 - 24 \hat{n} \cdot \vec{S}_1 \hat{n} \cdot \vec{S}_1 \vec{v}_2 \cdot \vec{a}_2 - 2 \vec{a}_1 \cdot \vec{v}_2 \vec{S}_1^2 + 2 \vec{v}_1 \cdot \vec{v}_2 \vec{S}_1^2 - \frac{1}{2} \vec{v}_2 \cdot \vec{v}_2 \vec{S}_1^2 \Bigg) + \frac{2 \hat{n} \cdot \vec{v}_2 \vec{S}_1^3}{r} \Bigg) m_2^2 C_{ES^2 1} \Bigg\}$$

{DiagS1CES2[3, 1, 1],

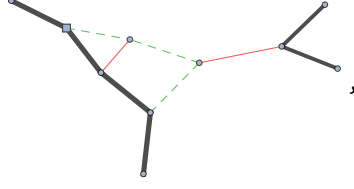

$$G^3 m_1 m_2 C_{ES^2 1} \left\{ \frac{-16 \vec{v}_1 \cdot \vec{v}_1 (\hat{n} \cdot \vec{S}_1)^2 - \frac{48}{7} \hat{n} \cdot \vec{S}_1 \hat{n} \cdot \vec{v}_1 \vec{S}_1 \cdot \vec{v}_1 + \frac{16}{7} \vec{S}_1 \cdot \vec{S}_1 (\hat{n} \cdot \vec{v}_1)^2 + \frac{16}{7} (\vec{S}_1 \cdot \vec{v}_1)^2 + \frac{32}{7} \vec{S}_1 \cdot \vec{S}_1 \vec{v}_1 \cdot \vec{v}_1}{r^5} + \frac{\frac{48}{5} \hat{n} \cdot \vec{S}_1 \vec{S}_1 \cdot \vec{v}_1 - \frac{32}{5} \vec{S}_1 \cdot \vec{S}_1 \hat{n} \cdot \vec{v}_1 + \frac{48}{5} \hat{n} \cdot \vec{S}_1 \vec{S}_1 \cdot \vec{v}_1}{r^4} \right\}$$

{DiagS1CES2[3, 1, 2],

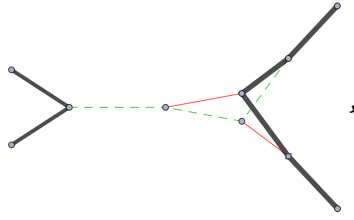

$$\frac{1}{r^5} G^3 m_1 m_2 C_{ES^2 1} \left( 32 \vec{v}_1 \cdot \vec{v}_2 (\hat{n} \cdot \vec{S}_1)^2 + \frac{80}{7} \hat{n} \cdot \vec{S}_1 \hat{n} \cdot \vec{v}_2 \vec{S}_1 \cdot \vec{v}_1 - \frac{128}{7} \hat{n} \cdot \vec{S}_1 \hat{n} \cdot \vec{v}_1 \vec{S}_1 \cdot \vec{v}_2 + \frac{16}{7} \vec{S}_1 \cdot \vec{S}_1 \hat{n} \cdot \vec{v}_1 \hat{n} \cdot \vec{v}_2 + \frac{16}{7} \vec{S}_1 \cdot \vec{v}_1 \vec{S}_1 \cdot \vec{v}_2 - \frac{80}{7} \vec{S}_1 \cdot \vec{S}_1 \vec{v}_1 \cdot \vec{v}_2 \right) \Bigg\}$$

{DiagS1CES2[3, 1, 3],

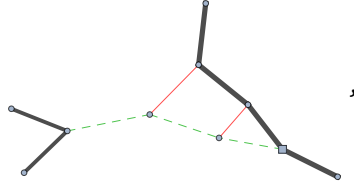

$$G^3 m_1 m_2 C_{ES^2 1} \left\{ \frac{1}{r^5} \left( \frac{256}{7} \vec{v}_1 \cdot \vec{v}_2 (\hat{n} \cdot \vec{S}_1)^2 - \frac{176}{7} \hat{n} \cdot \vec{S}_1 \hat{n} \cdot \vec{v}_2 \vec{S}_1 \cdot \vec{v}_1 + 32 \hat{n} \cdot \vec{S}_1 \hat{n} \cdot \vec{v}_1 \vec{S}_1 \cdot \vec{v}_2 - \frac{16}{7} \vec{S}_1 \cdot \vec{S}_1 \hat{n} \cdot \vec{v}_1 \hat{n} \cdot \vec{v}_2 - \frac{16}{7} \vec{S}_1 \cdot \vec{v}_1 \vec{S}_1 \cdot \vec{v}_2 - \frac{80}{7} \vec{S}_1 \cdot \vec{S}_1 \vec{v}_1 \cdot \vec{v}_2 \right) + \frac{-\frac{96}{5} \hat{n} \cdot \vec{S}_1 \vec{S}_1 \cdot \vec{v}_2 + \frac{64}{5} \vec{S}_1 \cdot \vec{S}_1 \hat{n} \cdot \vec{v}_2 - \frac{96}{5} \hat{n} \cdot \vec{S}_1 \vec{S}_1 \cdot \vec{v}_2}{r^4} \right\}$$

{DiagS1CES2[3, 1, 4],

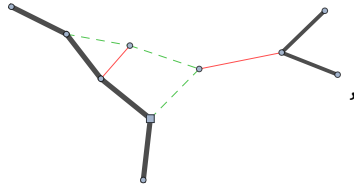

$$G^3 m_1 m_2 C_{ES^2 1} \left\{ \frac{\frac{48}{7} \vec{S}_1 \cdot \vec{S}_1 \vec{v}_1 \cdot \vec{v}_1 - \frac{144}{7} \vec{v}_1 \cdot \vec{v}_1 (\hat{n} \cdot \vec{S}_1)^2}{r^5} + \frac{\frac{48}{5} \hat{n} \cdot \vec{S}_1 \vec{S}_1 \cdot \vec{v}_1 - \frac{32}{5} \vec{S}_1 \cdot \vec{S}_1 \hat{n} \cdot \vec{v}_1 + \frac{48}{5} \hat{n} \cdot \vec{S}_1 \vec{S}_1 \cdot \vec{v}_1}{r^4} \right\}$$

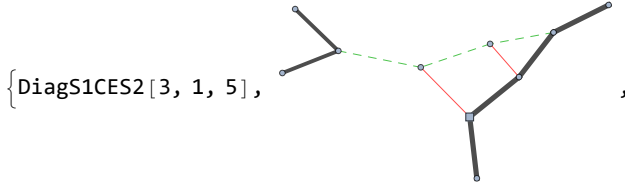

$$\frac{G^3 m_1 m_2 C_{ES^2 1} \left( \frac{192}{7} \vec{v}_1 \cdot \vec{v}_2 (\hat{n} \cdot \vec{S}_1)^2 + \frac{96}{7} \hat{n} \cdot \vec{S}_1 \hat{n} \cdot \vec{v}_2 \vec{S}_1 \cdot \vec{v}_1 - \frac{96}{7} \hat{n} \cdot \vec{S}_1 \hat{n} \cdot \vec{v}_1 \vec{S}_1 \cdot \vec{v}_2 - \frac{64}{7} \vec{S}_1 \cdot \vec{S}_1 \vec{v}_1 \cdot \vec{v}_2 \right)}{r^5}$$

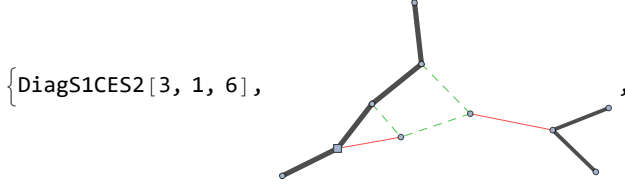

$$\frac{G^3 m_1 m_2 C_{ES^2 1} \left( -\frac{80}{7} \vec{v}_1 \cdot \vec{v}_1 (\hat{n} \cdot \vec{S}_1)^2 + \frac{48}{7} \hat{n} \cdot \vec{S}_1 \hat{n} \cdot \vec{v}_1 \vec{S}_1 \cdot \vec{v}_1 - \frac{16}{7} \vec{S}_1 \cdot \vec{S}_1 (\hat{n} \cdot \vec{v}_1)^2 - \frac{16}{7} (\vec{S}_1 \cdot \vec{v}_1)^2 + \frac{32}{7} \vec{S}_1 \cdot \vec{S}_1 \vec{v}_1 \cdot \vec{v}_1 \right)}{r^5}$$

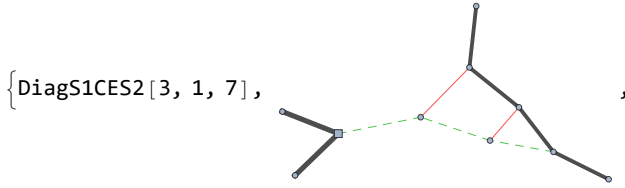

$$\frac{G^3 m_2^3 C_{ES^2 1} \left( \frac{160 \vec{v}_1 \cdot \vec{v}_2 (\hat{n} \cdot \vec{S}_1)^2 - 96 \vec{S}_1 \cdot \vec{S}_1 \vec{v}_1 \cdot \vec{v}_2}{r^5} + \frac{-32 \hat{n} \cdot \vec{S}_1 \vec{S}_1 \cdot \vec{v}_2 + 64 \vec{S}_1 \cdot \vec{S}_1 \hat{n} \cdot \vec{v}_2 - 32 \hat{n} \cdot \vec{S}_1 \vec{S}_1 \cdot \vec{v}_2}{r^4} \right)}{m_1}$$

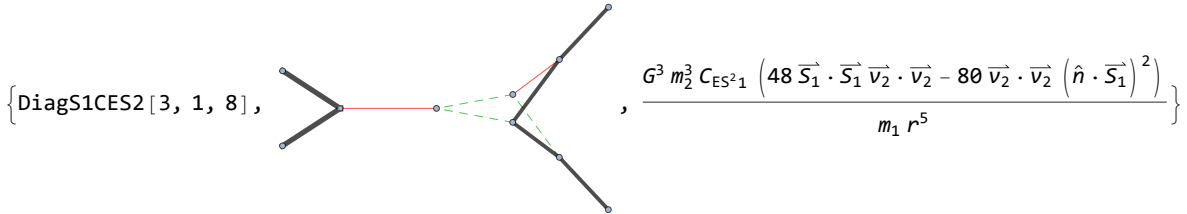

$$\frac{G^3 m_2^3 C_{ES^2 1} \left( 48 \vec{S}_1 \cdot \vec{S}_1 \vec{v}_2 \cdot \vec{v}_2 - 80 \vec{v}_2 \cdot \vec{v}_2 (\hat{n} \cdot \vec{S}_1)^2 \right)}{m_1 r^5}$$

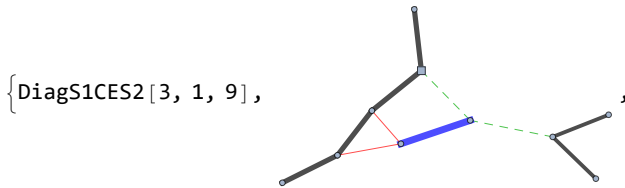

$$G^3 m_1 m_2 \left\{ \frac{-\frac{184}{49} \hat{n} \cdot \vec{S}_1 \hat{n} \cdot \vec{S}_1 \hat{n} \cdot \vec{v}_2 + \frac{4756 \vec{S}_1 \cdot \vec{S}_1 \hat{n} \cdot \vec{v}_2}{1225} + \frac{206 \hat{n} \cdot \vec{S}_1 \vec{S}_1 \cdot \vec{v}_2}{1225} + \frac{206 \hat{n} \cdot \vec{S}_1 \vec{S}_1 \cdot \vec{v}_2}{1225}}{r^4} + \right.$$

$$\left. \frac{1}{r^5} \left( \frac{16}{3} \hat{n} \cdot \vec{v}_1 \hat{n} \cdot \vec{v}_2 (\hat{n} \cdot \vec{S}_1)^2 + \frac{286}{147} \vec{v}_1 \cdot \vec{v}_2 (\hat{n} \cdot \vec{S}_1)^2 + \frac{68}{147} \hat{n} \cdot \vec{v}_2 \vec{S}_1 \cdot \vec{v}_1 \hat{n} \cdot \vec{S}_1 - \right. \right.$$



$$\begin{aligned}
& \left. \frac{184}{147} \hat{n} \cdot \vec{v}_1 \vec{S}_1 \cdot \vec{v}_2 \hat{n} \cdot \vec{S}_1 - \frac{232}{147} \hat{n} \cdot \vec{v}_1 \hat{n} \cdot \vec{v}_2 \vec{S}_1 \cdot \vec{S}_1 + \frac{136 \vec{S}_1 \cdot \vec{v}_1 \vec{S}_1 \cdot \vec{v}_2}{3675} - \frac{794 \vec{S}_1 \cdot \vec{S}_1 \vec{v}_1 \cdot \vec{v}_2}{1225} \right) + \\
& \left( \frac{\frac{12}{7} \hat{n} \cdot \vec{S}_1 \hat{n} \cdot \vec{S}_1 \hat{n} \cdot \vec{v}_2 - \frac{12}{35} \vec{S}_1 \cdot \vec{S}_1 \hat{n} \cdot \vec{v}_2 - \frac{12}{35} \hat{n} \cdot \vec{S}_1 \vec{S}_1 \cdot \vec{v}_2 - \frac{12}{35} \hat{n} \cdot \vec{S}_1 \vec{S}_1 \cdot \vec{v}_2}{r^4} + \frac{1}{r^5} \right. \\
& \quad \left( -2 \hat{n} \cdot \vec{v}_1 \hat{n} \cdot \vec{v}_2 (\hat{n} \cdot \vec{S}_1)^2 + \frac{2}{7} \vec{v}_1 \cdot \vec{v}_2 (\hat{n} \cdot \vec{S}_1)^2 + \frac{4}{7} \hat{n} \cdot \vec{v}_2 \vec{S}_1 \cdot \vec{v}_1 \hat{n} \cdot \vec{S}_1 + \frac{4}{7} \hat{n} \cdot \vec{v}_1 \vec{S}_1 \cdot \vec{v}_2 \hat{n} \cdot \vec{S}_1 + \right. \\
& \quad \left. \frac{2}{7} \hat{n} \cdot \vec{v}_1 \hat{n} \cdot \vec{v}_2 \vec{S}_1 \cdot \vec{S}_1 - \frac{4}{35} \vec{S}_1 \cdot \vec{v}_1 \vec{S}_1 \cdot \vec{v}_2 - \frac{2}{35} \vec{S}_1 \cdot \vec{S}_1 \vec{v}_1 \cdot \vec{v}_2 \right) \log \left( \frac{r}{R_\theta} \right) + \\
& \quad \left. \frac{1}{\epsilon_d} \left( \frac{-\frac{4}{7} \hat{n} \cdot \vec{S}_1 \hat{n} \cdot \vec{S}_1 \hat{n} \cdot \vec{v}_2 + \frac{4}{35} \vec{S}_1 \cdot \vec{S}_1 \hat{n} \cdot \vec{v}_2 + \frac{4}{35} \hat{n} \cdot \vec{S}_1 \vec{S}_1 \cdot \vec{v}_2 + \frac{4}{35} \hat{n} \cdot \vec{S}_1 \vec{S}_1 \cdot \vec{v}_2}{r^4} + \frac{1}{r^5} \right. \right. \\
& \quad \left( \frac{2}{3} \hat{n} \cdot \vec{v}_1 \hat{n} \cdot \vec{v}_2 (\hat{n} \cdot \vec{S}_1)^2 - \frac{2}{21} \vec{v}_1 \cdot \vec{v}_2 (\hat{n} \cdot \vec{S}_1)^2 - \frac{4}{21} \hat{n} \cdot \vec{v}_2 \vec{S}_1 \cdot \vec{v}_1 \hat{n} \cdot \vec{S}_1 - \frac{4}{21} \hat{n} \cdot \vec{v}_1 \vec{S}_1 \cdot \vec{v}_2 \hat{n} \cdot \vec{S}_1 - \right. \\
& \quad \left. \left. \frac{2}{21} \hat{n} \cdot \vec{v}_1 \hat{n} \cdot \vec{v}_2 \vec{S}_1 \cdot \vec{S}_1 + \frac{4}{105} \vec{S}_1 \cdot \vec{v}_1 \vec{S}_1 \cdot \vec{v}_2 + \frac{2}{105} \vec{S}_1 \cdot \vec{S}_1 \vec{v}_1 \cdot \vec{v}_2 \right) \right) \Bigg\} C_{ES^2_1} \}
\end{aligned}$$

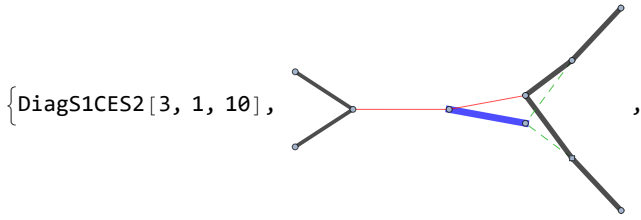

$$\begin{aligned}
& G^3 m_1 m_2 C_{ES^2_1} \left( \frac{1}{\epsilon_d} \left( \frac{1}{r^5} \left( -12 (\hat{n} \cdot \vec{S}_1)^2 (\hat{n} \cdot \vec{v}_1)^2 + \frac{12}{7} \vec{v}_1 \cdot \vec{v}_1 (\hat{n} \cdot \vec{S}_1)^2 + \frac{48}{7} \hat{n} \cdot \vec{S}_1 \hat{n} \cdot \vec{v}_1 \vec{S}_1 \cdot \vec{v}_1 + \frac{12}{7} \vec{S}_1 \cdot \vec{S}_1 (\hat{n} \cdot \vec{v}_1)^2 - \right. \right. \right. \\
& \quad \left. \left. \frac{24}{35} (\vec{S}_1 \cdot \vec{v}_1)^2 - \frac{12}{35} \vec{S}_1 \cdot \vec{S}_1 \vec{v}_1 \cdot \vec{v}_1 \right) + \frac{8 \hat{n} \cdot \vec{S}_1 \hat{n} \cdot \vec{S}_1 \hat{n} \cdot \vec{v}_1 - \frac{8}{5} \vec{S}_1 \cdot \vec{S}_1 \hat{n} \cdot \vec{v}_1 - \frac{8}{5} \hat{n} \cdot \vec{S}_1 \vec{S}_1 \cdot \vec{v}_1 - \frac{8}{5} \hat{n} \cdot \vec{S}_1 \vec{S}_1 \cdot \vec{v}_1}{r^4} \right) + \right. \\
& \quad \left. \frac{1}{r^5} \left( -34 (\hat{n} \cdot \vec{S}_1)^2 (\hat{n} \cdot \vec{v}_1)^2 + \frac{286}{49} \vec{v}_1 \cdot \vec{v}_1 (\hat{n} \cdot \vec{S}_1)^2 + \frac{640}{49} \hat{n} \cdot \vec{S}_1 \hat{n} \cdot \vec{v}_1 \vec{S}_1 \cdot \vec{v}_1 + \right. \right. \\
& \quad \left. \left. \frac{398}{49} \vec{S}_1 \cdot \vec{S}_1 (\hat{n} \cdot \vec{v}_1)^2 - \frac{676}{1225} (\vec{S}_1 \cdot \vec{v}_1)^2 - \frac{2438 \vec{S}_1 \cdot \vec{S}_1 \vec{v}_1 \cdot \vec{v}_1}{1225} \right) + \right. \\
& \quad \left. \frac{20 \hat{n} \cdot \vec{S}_1 \hat{n} \cdot \vec{S}_1 \hat{n} \cdot \vec{v}_1 - \frac{176}{25} \vec{S}_1 \cdot \vec{S}_1 \hat{n} \cdot \vec{v}_1 - \frac{66}{25} \hat{n} \cdot \vec{S}_1 \vec{S}_1 \cdot \vec{v}_1 - \frac{66}{25} \hat{n} \cdot \vec{S}_1 \vec{S}_1 \cdot \vec{v}_1}{r^4} + \log \left( \frac{r}{R_\theta} \right) \right. \\
& \quad \left. \left( \frac{1}{r^5} \left( 36 (\hat{n} \cdot \vec{S}_1)^2 (\hat{n} \cdot \vec{v}_1)^2 - \frac{36}{7} \vec{v}_1 \cdot \vec{v}_1 (\hat{n} \cdot \vec{S}_1)^2 - \frac{144}{7} \hat{n} \cdot \vec{S}_1 \hat{n} \cdot \vec{v}_1 \vec{S}_1 \cdot \vec{v}_1 - \frac{36}{7} \vec{S}_1 \cdot \vec{S}_1 (\hat{n} \cdot \vec{v}_1)^2 + \frac{72}{35} (\vec{S}_1 \cdot \vec{v}_1)^2 + \right. \right. \right.
\end{aligned}$$

$$\left. \left. \frac{36}{35} \vec{S}_1 \cdot \vec{S}_1 \vec{v}_1 \cdot \vec{v}_1 \right) + \frac{-24 \hat{n} \cdot \vec{S}_1 \hat{n} \cdot \vec{S}_1 \hat{n} \cdot \vec{v}_1 + \frac{24}{5} \vec{S}_1 \cdot \vec{S}_1 \hat{n} \cdot \vec{v}_1 + \frac{24}{5} \hat{n} \cdot \vec{S}_1 \vec{S}_1 \cdot \vec{v}_1 + \frac{24}{5} \hat{n} \cdot \vec{S}_1 \vec{S}_1 \cdot \vec{v}_1}{r^4} \right) \right\}$$

{DiagS1CES2[3, 1, 11],

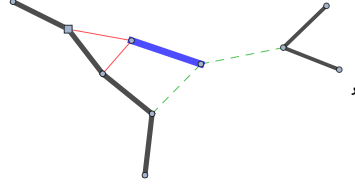

$$\begin{aligned} G^3 m_1 m_2 C_{ES^2 1} \left( \frac{1}{r^5 \in_d} \left( \frac{20}{3} \left( \hat{n} \cdot \vec{S}_1 \right)^2 \hat{n} \cdot \vec{v}_1 \hat{n} \cdot \vec{v}_2 - \frac{20}{21} \vec{v}_1 \cdot \vec{v}_2 \left( \hat{n} \cdot \vec{S}_1 \right)^2 - \frac{40}{21} \hat{n} \cdot \vec{S}_1 \hat{n} \cdot \vec{v}_2 \vec{S}_1 \cdot \vec{v}_1 - \right. \right. \\ \left. \frac{40}{21} \hat{n} \cdot \vec{S}_1 \hat{n} \cdot \vec{v}_1 \vec{S}_1 \cdot \vec{v}_2 - \frac{20}{21} \vec{S}_1 \cdot \vec{S}_1 \hat{n} \cdot \vec{v}_1 \hat{n} \cdot \vec{v}_2 + \frac{8}{21} \vec{S}_1 \cdot \vec{v}_1 \vec{S}_1 \cdot \vec{v}_2 + \frac{4}{21} \vec{S}_1 \cdot \vec{S}_1 \vec{v}_1 \cdot \vec{v}_2 \right) + \\ \left. \frac{1}{r^5} \log \left( \frac{r}{R_0} \right) \left( -20 \left( \hat{n} \cdot \vec{S}_1 \right)^2 \hat{n} \cdot \vec{v}_1 \hat{n} \cdot \vec{v}_2 + \frac{20}{7} \vec{v}_1 \cdot \vec{v}_2 \left( \hat{n} \cdot \vec{S}_1 \right)^2 + \frac{40}{7} \hat{n} \cdot \vec{S}_1 \hat{n} \cdot \vec{v}_2 \vec{S}_1 \cdot \vec{v}_1 + \right. \right. \\ \left. \frac{40}{7} \hat{n} \cdot \vec{S}_1 \hat{n} \cdot \vec{v}_1 \vec{S}_1 \cdot \vec{v}_2 + \frac{20}{7} \vec{S}_1 \cdot \vec{S}_1 \hat{n} \cdot \vec{v}_1 \hat{n} \cdot \vec{v}_2 - \frac{8}{7} \vec{S}_1 \cdot \vec{v}_1 \vec{S}_1 \cdot \vec{v}_2 - \frac{4}{7} \vec{S}_1 \cdot \vec{S}_1 \vec{v}_1 \cdot \vec{v}_2 \right) + \frac{1}{r^5} \\ \left. \left( 33 \left( \hat{n} \cdot \vec{S}_1 \right)^2 \hat{n} \cdot \vec{v}_1 \hat{n} \cdot \vec{v}_2 - \frac{661}{147} \vec{v}_1 \cdot \vec{v}_2 \left( \hat{n} \cdot \vec{S}_1 \right)^2 - \frac{1658}{147} \hat{n} \cdot \vec{S}_1 \hat{n} \cdot \vec{v}_2 \vec{S}_1 \cdot \vec{v}_1 - \frac{1322}{147} \hat{n} \cdot \vec{S}_1 \hat{n} \cdot \vec{v}_1 \vec{S}_1 \cdot \vec{v}_2 - \right. \right. \\ \left. \left. \frac{239}{49} \vec{S}_1 \cdot \vec{S}_1 \hat{n} \cdot \vec{v}_1 \hat{n} \cdot \vec{v}_2 + \frac{118}{49} \vec{S}_1 \cdot \vec{v}_1 \vec{S}_1 \cdot \vec{v}_2 + \frac{121}{147} \vec{S}_1 \cdot \vec{S}_1 \vec{v}_1 \cdot \vec{v}_2 \right) \right) \right\} \end{aligned}$$

{DiagS1CES2[3, 1, 12],

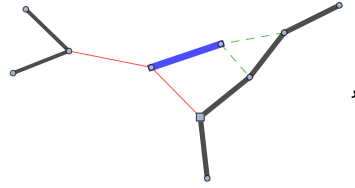

$$\begin{aligned} G^3 m_1 m_2 C_{ES^2 1} \left( \frac{1}{r^5 \in_d} \left( -30 \left( \hat{n} \cdot \vec{S}_1 \right)^2 \left( \hat{n} \cdot \vec{v}_1 \right)^2 + \frac{30}{7} \vec{v}_1 \cdot \vec{v}_1 \left( \hat{n} \cdot \vec{S}_1 \right)^2 + \right. \right. \\ \left. \frac{120}{7} \hat{n} \cdot \vec{S}_1 \hat{n} \cdot \vec{v}_1 \vec{S}_1 \cdot \vec{v}_1 + \frac{30}{7} \vec{S}_1 \cdot \vec{S}_1 \left( \hat{n} \cdot \vec{v}_1 \right)^2 - \frac{12}{7} \left( \vec{S}_1 \cdot \vec{v}_1 \right)^2 - \frac{6}{7} \vec{S}_1 \cdot \vec{S}_1 \vec{v}_1 \cdot \vec{v}_1 \right) + \frac{1}{r^5} \\ \log \left( \frac{r}{R_0} \right) \left( 90 \left( \hat{n} \cdot \vec{S}_1 \right)^2 \left( \hat{n} \cdot \vec{v}_1 \right)^2 - \frac{90}{7} \vec{v}_1 \cdot \vec{v}_1 \left( \hat{n} \cdot \vec{S}_1 \right)^2 - \frac{360}{7} \hat{n} \cdot \vec{S}_1 \hat{n} \cdot \vec{v}_1 \vec{S}_1 \cdot \vec{v}_1 - \frac{90}{7} \vec{S}_1 \cdot \vec{S}_1 \left( \hat{n} \cdot \vec{v}_1 \right)^2 + \right. \\ \left. \frac{36}{7} \left( \vec{S}_1 \cdot \vec{v}_1 \right)^2 + \frac{18}{7} \vec{S}_1 \cdot \vec{S}_1 \vec{v}_1 \cdot \vec{v}_1 \right) + \frac{1}{r^5} \left( -61 \left( \hat{n} \cdot \vec{S}_1 \right)^2 \left( \hat{n} \cdot \vec{v}_1 \right)^2 + \frac{589}{49} \vec{v}_1 \cdot \vec{v}_1 \left( \hat{n} \cdot \vec{S}_1 \right)^2 + \right. \\ \left. \frac{1516}{49} \hat{n} \cdot \vec{S}_1 \hat{n} \cdot \vec{v}_1 \vec{S}_1 \cdot \vec{v}_1 + \frac{631}{49} \vec{S}_1 \cdot \vec{S}_1 \left( \hat{n} \cdot \vec{v}_1 \right)^2 - \frac{118}{49} \left( \vec{S}_1 \cdot \vec{v}_1 \right)^2 - \frac{185}{49} \vec{S}_1 \cdot \vec{S}_1 \vec{v}_1 \cdot \vec{v}_1 \right) \right) \right\} \end{aligned}$$

{DiagS1CES2[3, 1, 13],

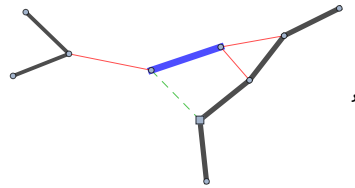

$$\begin{aligned} G^3 m_1 m_2 \left( \frac{\frac{63}{25} \left( \hat{n} \cdot \vec{S}_1 \right)^2 + \frac{63}{25} \hat{n} \cdot \vec{S}_1 \hat{n} \cdot \vec{S}_1 - \frac{143}{75} \vec{S}_1 \cdot \vec{S}_1 - \frac{143}{75} \vec{S}_1 \cdot \vec{S}_1}{r^3} + \frac{1}{r^4} \left( -\frac{429}{98} \hat{n} \cdot \vec{a}_1 \left( \hat{n} \cdot \vec{S}_1 \right)^2 - \right. \right. \\ \left. \frac{858}{49} \hat{n} \cdot \vec{S}_1 \hat{n} \cdot \vec{v}_1 \hat{n} \cdot \vec{S}_1 + 15 \hat{n} \cdot \vec{S}_1 \hat{n} \cdot \vec{v}_2 \hat{n} \cdot \vec{S}_1 + \frac{3009}{1225} \vec{S}_1 \cdot \vec{v}_1 \hat{n} \cdot \vec{S}_1 - \frac{63}{25} \vec{S}_1 \cdot \vec{v}_2 \hat{n} \cdot \vec{S}_1 + \frac{1137}{1225} \vec{S}_1 \cdot \vec{a}_1 \hat{n} \cdot \vec{S}_1 + \right. \end{aligned}$$

$$\begin{aligned}
& \left. \frac{7944 \hat{n} \cdot \vec{v}_1 \vec{S}_1 \cdot \vec{S}_1^{\frac{1}{2}}}{1225} - \frac{163}{25} \hat{n} \cdot \vec{v}_2 \vec{S}_1 \cdot \vec{S}_1^{\frac{1}{2}} + \frac{3237 \hat{n} \cdot \vec{a}_1 \vec{S}_1 \cdot \vec{S}_1^{\frac{1}{2}}}{2450} + \frac{3009 \hat{n} \cdot \vec{S}_1 \vec{S}_1 \cdot \vec{v}_1}{1225} - \frac{63}{25} \hat{n} \cdot \vec{S}_1 \vec{S}_1 \cdot \vec{v}_2 \right) + \\
& \frac{1}{r^5} \left( \frac{143}{6} (\hat{n} \cdot \vec{v}_1)^2 (\hat{n} \cdot \vec{S}_1)^2 - \frac{69}{2} \hat{n} \cdot \vec{v}_1 \hat{n} \cdot \vec{v}_2 (\hat{n} \cdot \vec{S}_1)^2 - \frac{601}{294} \vec{v}_1 \cdot \vec{v}_1 (\hat{n} \cdot \vec{S}_1)^2 + \frac{429}{98} \vec{v}_1 \cdot \vec{v}_2 (\hat{n} \cdot \vec{S}_1)^2 - \right. \\
& \frac{1706}{147} \hat{n} \cdot \vec{v}_1 \vec{S}_1 \cdot \vec{v}_1 \hat{n} \cdot \vec{S}_1 + \frac{303}{49} \hat{n} \cdot \vec{v}_2 \vec{S}_1 \cdot \vec{v}_1 \hat{n} \cdot \vec{S}_1 + \frac{429}{49} \hat{n} \cdot \vec{v}_1 \vec{S}_1 \cdot \vec{v}_2 \hat{n} \cdot \vec{S}_1 + \frac{109}{147} (\vec{S}_1 \cdot \vec{v}_1)^2 - \\
& \left. \frac{1385}{294} (\hat{n} \cdot \vec{v}_1)^2 \vec{S}_1 \cdot \vec{S}_1 + \frac{723}{98} \hat{n} \cdot \vec{v}_1 \hat{n} \cdot \vec{v}_2 \vec{S}_1 \cdot \vec{S}_1 - \frac{1137 \vec{S}_1 \cdot \vec{v}_1 \vec{S}_1 \cdot \vec{v}_2}{1225} + \frac{55}{98} \vec{S}_1 \cdot \vec{S}_1 \vec{v}_1 \cdot \vec{v}_1 - \frac{3237 \vec{S}_1 \cdot \vec{S}_1 \vec{v}_1 \cdot \vec{v}_2}{2450} \right) + \\
& \left( \frac{-\frac{12}{5} \left( \hat{n} \cdot \vec{S}_1^{\frac{1}{2}} \right)^2 - \frac{12}{5} \hat{n} \cdot \vec{S}_1^{\frac{2}{2}} \hat{n} \cdot \vec{S}_1 + \frac{4}{5} \vec{S}_1 \cdot \vec{S}_1^{\frac{1}{2}} + \frac{4}{5} \vec{S}_1 \cdot \vec{S}_1^{\frac{2}{2}}}{r^3} + \frac{1}{r^4} \left( \frac{27}{7} \hat{n} \cdot \vec{a}_1 (\hat{n} \cdot \vec{S}_1)^2 + \frac{108}{7} \hat{n} \cdot \vec{S}_1 \hat{n} \cdot \vec{v}_1 \hat{n} \cdot \vec{S}_1 - \right. \right. \\
& 12 \hat{n} \cdot \vec{S}_1^{\frac{1}{2}} \hat{n} \cdot \vec{v}_2 \hat{n} \cdot \vec{S}_1 - \frac{108}{35} \vec{S}_1 \cdot \vec{v}_1 \hat{n} \cdot \vec{S}_1 + \frac{12}{5} \vec{S}_1 \cdot \vec{v}_2 \hat{n} \cdot \vec{S}_1 - \frac{54}{35} \vec{S}_1 \cdot \vec{a}_1 \hat{n} \cdot \vec{S}_1 - \frac{108}{35} \hat{n} \cdot \vec{v}_1 \vec{S}_1 \cdot \vec{S}_1^{\frac{1}{2}} + \\
& \left. \frac{12}{5} \hat{n} \cdot \vec{v}_2 \vec{S}_1 \cdot \vec{S}_1^{\frac{1}{2}} - \frac{27}{35} \hat{n} \cdot \vec{a}_1 \vec{S}_1 \cdot \vec{S}_1 - \frac{108}{35} \hat{n} \cdot \vec{S}_1 \vec{S}_1 \cdot \vec{v}_1 + \frac{12}{5} \hat{n} \cdot \vec{S}_1 \vec{S}_1 \cdot \vec{v}_2 \right) + \frac{1}{r^5} \\
& \left( -20 (\hat{n} \cdot \vec{v}_1)^2 (\hat{n} \cdot \vec{S}_1)^2 + 27 \hat{n} \cdot \vec{v}_1 \hat{n} \cdot \vec{v}_2 (\hat{n} \cdot \vec{S}_1)^2 + \frac{20}{7} \vec{v}_1 \cdot \vec{v}_1 (\hat{n} \cdot \vec{S}_1)^2 - \frac{27}{7} \vec{v}_1 \cdot \vec{v}_2 (\hat{n} \cdot \vec{S}_1)^2 + \right. \\
& \frac{80}{7} \hat{n} \cdot \vec{v}_1 \vec{S}_1 \cdot \vec{v}_1 \hat{n} \cdot \vec{S}_1 - \frac{54}{7} \hat{n} \cdot \vec{v}_2 \vec{S}_1 \cdot \vec{v}_1 \hat{n} \cdot \vec{S}_1 - \frac{54}{7} \hat{n} \cdot \vec{v}_1 \vec{S}_1 \cdot \vec{v}_2 \hat{n} \cdot \vec{S}_1 - \frac{8}{7} (\vec{S}_1 \cdot \vec{v}_1)^2 + \\
& \left. \frac{20}{7} (\hat{n} \cdot \vec{v}_1)^2 \vec{S}_1 \cdot \vec{S}_1 - \frac{27}{7} \hat{n} \cdot \vec{v}_1 \hat{n} \cdot \vec{v}_2 \vec{S}_1 \cdot \vec{S}_1 + \frac{54}{35} \vec{S}_1 \cdot \vec{v}_1 \vec{S}_1 \cdot \vec{v}_2 - \frac{4}{7} \vec{S}_1 \cdot \vec{S}_1 \vec{v}_1 \cdot \vec{v}_1 + \frac{27}{35} \vec{S}_1 \cdot \vec{S}_1 \vec{v}_1 \cdot \vec{v}_2 \right) \Bigg) \\
& \log \left( \frac{r}{R_\theta} \right) + \frac{1}{\epsilon_d} \left( \frac{\frac{4}{5} \left( \hat{n} \cdot \vec{S}_1^{\frac{1}{2}} \right)^2 + \frac{4}{5} \hat{n} \cdot \vec{S}_1^{\frac{2}{2}} \hat{n} \cdot \vec{S}_1 - \frac{4}{15} \vec{S}_1 \cdot \vec{S}_1^{\frac{1}{2}} - \frac{4}{15} \vec{S}_1 \cdot \vec{S}_1^{\frac{2}{2}}}{r^3} + \frac{1}{r^4} \right. \\
& \left( -\frac{9}{7} \hat{n} \cdot \vec{a}_1 (\hat{n} \cdot \vec{S}_1)^2 - \frac{36}{7} \hat{n} \cdot \vec{S}_1 \hat{n} \cdot \vec{v}_1 \hat{n} \cdot \vec{S}_1 + 4 \hat{n} \cdot \vec{S}_1 \hat{n} \cdot \vec{v}_2 \hat{n} \cdot \vec{S}_1 + \frac{36}{35} \vec{S}_1 \cdot \vec{v}_1 \hat{n} \cdot \vec{S}_1 - \frac{4}{5} \vec{S}_1 \cdot \vec{v}_2 \hat{n} \cdot \vec{S}_1 + \right. \\
& \frac{18}{35} \vec{S}_1 \cdot \vec{a}_1 \hat{n} \cdot \vec{S}_1 + \frac{36}{35} \hat{n} \cdot \vec{v}_1 \vec{S}_1 \cdot \vec{S}_1^{\frac{1}{2}} - \frac{4}{5} \hat{n} \cdot \vec{v}_2 \vec{S}_1 \cdot \vec{S}_1^{\frac{1}{2}} + \frac{9}{35} \hat{n} \cdot \vec{a}_1 \vec{S}_1 \cdot \vec{S}_1 + \frac{36}{35} \hat{n} \cdot \vec{S}_1 \vec{S}_1 \cdot \vec{v}_1 - \frac{4}{5} \hat{n} \cdot \vec{S}_1 \vec{S}_1 \cdot \vec{v}_2 \Bigg) + \\
& \frac{1}{r^5} \left( \frac{20}{3} (\hat{n} \cdot \vec{v}_1)^2 (\hat{n} \cdot \vec{S}_1)^2 - 9 \hat{n} \cdot \vec{v}_1 \hat{n} \cdot \vec{v}_2 (\hat{n} \cdot \vec{S}_1)^2 - \frac{20}{21} \vec{v}_1 \cdot \vec{v}_1 (\hat{n} \cdot \vec{S}_1)^2 + \frac{9}{7} \vec{v}_1 \cdot \vec{v}_2 (\hat{n} \cdot \vec{S}_1)^2 - \right. \\
& \frac{80}{21} \hat{n} \cdot \vec{v}_1 \vec{S}_1 \cdot \vec{v}_1 \hat{n} \cdot \vec{S}_1 + \frac{18}{7} \hat{n} \cdot \vec{v}_2 \vec{S}_1 \cdot \vec{v}_1 \hat{n} \cdot \vec{S}_1 + \frac{18}{7} \hat{n} \cdot \vec{v}_1 \vec{S}_1 \cdot \vec{v}_2 \hat{n} \cdot \vec{S}_1 + \frac{8}{21} (\vec{S}_1 \cdot \vec{v}_1)^2 - \frac{20}{21} (\hat{n} \cdot \vec{v}_1)^2 \vec{S}_1 \cdot \vec{S}_1 + \\
& \left. \left. \frac{9}{7} \hat{n} \cdot \vec{v}_1 \hat{n} \cdot \vec{v}_2 \vec{S}_1 \cdot \vec{S}_1 - \frac{18}{35} \vec{S}_1 \cdot \vec{v}_1 \vec{S}_1 \cdot \vec{v}_2 + \frac{4}{21} \vec{S}_1 \cdot \vec{S}_1 \vec{v}_1 \cdot \vec{v}_1 - \frac{9}{35} \vec{S}_1 \cdot \vec{S}_1 \vec{v}_1 \cdot \vec{v}_2 \right) \right) \Bigg\} c_{\text{ES}^2_1} \Bigg\}
\end{aligned}$$

{DiagS1CES2[3, 1, 14],

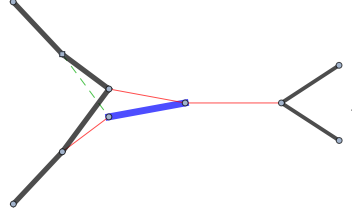

$$\begin{aligned}
 & G^3 m_1 m_2 \left( \frac{-\frac{4}{3} \frac{1}{S_1} \cdot \frac{1}{S_1} - \frac{4}{3} \frac{S_1}{S_1} \cdot \frac{2}{S_1}}{r^3} + \frac{1}{r^4} \left( 3 \hat{n} \cdot \vec{a}_1 \left( \hat{n} \cdot \vec{S}_1 \right)^2 + 14 \hat{n} \cdot \vec{S}_1 \hat{n} \cdot \vec{v}_1 \hat{n} \cdot \vec{S}_1 - \right. \right. \\
 & \quad \left. \frac{81}{25} \frac{1}{S_1} \cdot \vec{v}_1 \hat{n} \cdot \vec{S}_1 - \frac{38}{25} \vec{S}_1 \cdot \vec{a}_1 \hat{n} \cdot \vec{S}_1 - \frac{36}{25} \hat{n} \cdot \vec{v}_1 \vec{S}_1 \cdot \frac{1}{S_1} - \frac{19}{25} \hat{n} \cdot \vec{a}_1 \vec{S}_1 \cdot \vec{S}_1 - \frac{81}{25} \hat{n} \cdot \vec{S}_1 \vec{S}_1 \cdot \vec{v}_1 \right) + \\
 & \quad \frac{1}{r^5} \left( -20 \left( \hat{n} \cdot \vec{v}_1 \right)^2 \left( \hat{n} \cdot \vec{S}_1 \right)^2 + \frac{88}{49} \vec{v}_1 \cdot \vec{v}_1 \left( \hat{n} \cdot \vec{S}_1 \right)^2 + \frac{660}{49} \hat{n} \cdot \vec{v}_1 \vec{S}_1 \cdot \vec{v}_1 \hat{n} \cdot \vec{S}_1 - \frac{1524 \left( \vec{S}_1 \cdot \vec{v}_1 \right)^2}{1225} + \right. \\
 & \quad \left. \frac{144}{49} \left( \hat{n} \cdot \vec{v}_1 \right)^2 \vec{S}_1 \cdot \vec{S}_1 - \frac{412 \vec{S}_1 \cdot \vec{S}_1 \vec{v}_1 \cdot \vec{v}_1}{1225} \right) + \left( \frac{6 \left( \hat{n} \cdot \vec{S}_1 \right)^2 + 6 \hat{n} \cdot \vec{S}_1 \hat{n} \cdot \vec{S}_1 - 2 \vec{S}_1 \cdot \frac{1}{S_1} - 2 \vec{S}_1 \cdot \frac{2}{S_1}}{r^3} + \frac{1}{r^4} \right. \\
 & \quad \left( -6 \hat{n} \cdot \vec{a}_1 \left( \hat{n} \cdot \vec{S}_1 \right)^2 - 24 \hat{n} \cdot \vec{S}_1 \hat{n} \cdot \vec{v}_1 \hat{n} \cdot \vec{S}_1 + \frac{24}{5} \frac{1}{S_1} \cdot \vec{v}_1 \hat{n} \cdot \vec{S}_1 + \frac{12}{5} \vec{S}_1 \cdot \vec{a}_1 \hat{n} \cdot \vec{S}_1 + \frac{24}{5} \hat{n} \cdot \vec{v}_1 \vec{S}_1 \cdot \frac{1}{S_1} + \right. \\
 & \quad \left. \frac{6}{5} \hat{n} \cdot \vec{a}_1 \vec{S}_1 \cdot \vec{S}_1 + \frac{24}{5} \hat{n} \cdot \vec{S}_1 \vec{S}_1 \cdot \vec{v}_1 \right) + \frac{1}{r^5} \left( 24 \left( \hat{n} \cdot \vec{v}_1 \right)^2 \left( \hat{n} \cdot \vec{S}_1 \right)^2 - \frac{24}{7} \vec{v}_1 \cdot \vec{v}_1 \left( \hat{n} \cdot \vec{S}_1 \right)^2 - \right. \\
 & \quad \left. \frac{96}{7} \hat{n} \cdot \vec{v}_1 \vec{S}_1 \cdot \vec{v}_1 \hat{n} \cdot \vec{S}_1 + \frac{48}{35} \left( \vec{S}_1 \cdot \vec{v}_1 \right)^2 - \frac{24}{7} \left( \hat{n} \cdot \vec{v}_1 \right)^2 \vec{S}_1 \cdot \vec{S}_1 + \frac{24}{35} \vec{S}_1 \cdot \vec{S}_1 \vec{v}_1 \cdot \vec{v}_1 \right) \log \left( \frac{r}{R_0} \right) + \frac{1}{\epsilon_d} \\
 & \quad \left( \frac{-2 \left( \hat{n} \cdot \vec{S}_1 \right)^2 - 2 \hat{n} \cdot \vec{S}_1 \hat{n} \cdot \vec{S}_1 + \frac{2}{3} \frac{1}{S_1} \cdot \frac{1}{S_1} + \frac{2}{3} \vec{S}_1 \cdot \frac{2}{S_1}}{r^3} + \frac{1}{r^4} \left( 2 \hat{n} \cdot \vec{a}_1 \left( \hat{n} \cdot \vec{S}_1 \right)^2 + 8 \hat{n} \cdot \vec{S}_1 \hat{n} \cdot \vec{v}_1 \hat{n} \cdot \vec{S}_1 - \frac{8}{5} \frac{1}{S_1} \cdot \vec{v}_1 \hat{n} \cdot \vec{S}_1 - \right. \right. \\
 & \quad \left. \frac{4}{5} \vec{S}_1 \cdot \vec{a}_1 \hat{n} \cdot \vec{S}_1 - \frac{8}{5} \hat{n} \cdot \vec{v}_1 \vec{S}_1 \cdot \frac{1}{S_1} - \frac{2}{5} \hat{n} \cdot \vec{a}_1 \vec{S}_1 \cdot \vec{S}_1 - \frac{8}{5} \hat{n} \cdot \vec{S}_1 \vec{S}_1 \cdot \vec{v}_1 \right) + \frac{1}{r^5} \left( -8 \left( \hat{n} \cdot \vec{v}_1 \right)^2 \left( \hat{n} \cdot \vec{S}_1 \right)^2 + \right. \\
 & \quad \left. \frac{8}{7} \vec{v}_1 \cdot \vec{v}_1 \left( \hat{n} \cdot \vec{S}_1 \right)^2 + \frac{32}{7} \hat{n} \cdot \vec{v}_1 \vec{S}_1 \cdot \vec{v}_1 \hat{n} \cdot \vec{S}_1 - \frac{16}{35} \left( \vec{S}_1 \cdot \vec{v}_1 \right)^2 + \frac{8}{7} \left( \hat{n} \cdot \vec{v}_1 \right)^2 \vec{S}_1 \cdot \vec{S}_1 - \frac{8}{35} \vec{S}_1 \cdot \vec{S}_1 \vec{v}_1 \cdot \vec{v}_1 \right) \Bigg) \Bigg\} C_{ES^2_1}
 \end{aligned}$$

{DiagS1CES2[3, 1, 15],

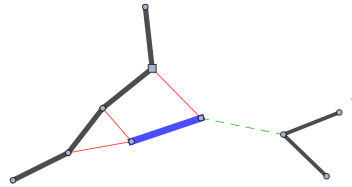

,  $G^3 m_1 m_2$

$$\begin{aligned}
& \left( \frac{429}{98} \hat{n} \cdot \vec{a}_2 \left( \hat{n} \cdot \vec{S}_1 \right)^2 + \frac{429}{49} \hat{n} \cdot \vec{S}_1 \hat{n} \cdot \vec{v}_2 \hat{n} \cdot \vec{S}_1 - \frac{1137 \vec{S}_1 \cdot \vec{v}_2 \hat{n} \cdot \vec{S}_1}{1225} - \frac{1137 \vec{S}_1 \cdot \vec{a}_2 \hat{n} \cdot \vec{S}_1}{1225} - \frac{3237 \hat{n} \cdot \vec{v}_2 \vec{S}_1 \cdot \vec{S}_1}{1225} - \frac{3237 \hat{n} \cdot \vec{a}_2 \vec{S}_1 \cdot \vec{S}_1}{2450} - \frac{1137 \hat{n} \cdot \vec{S}_1 \vec{S}_1 \cdot \vec{v}_2}{1225} \right. \\
& \quad \left. \frac{1}{r^4} \right. \\
& + \frac{1}{r^5} \left( \frac{69}{2} \left( \hat{n} \cdot \vec{v}_2 \right)^2 \left( \hat{n} \cdot \vec{S}_1 \right)^2 - \frac{143}{6} \hat{n} \cdot \vec{v}_1 \hat{n} \cdot \vec{v}_2 \left( \hat{n} \cdot \vec{S}_1 \right)^2 + \frac{601}{294} \vec{v}_1 \cdot \vec{v}_2 \left( \hat{n} \cdot \vec{S}_1 \right)^2 - \frac{429}{98} \vec{v}_2 \cdot \vec{v}_2 \left( \hat{n} \cdot \vec{S}_1 \right)^2 + \right. \\
& \quad \frac{1105}{147} \hat{n} \cdot \vec{v}_2 \vec{S}_1 \cdot \vec{v}_1 \hat{n} \cdot \vec{S}_1 + \frac{601}{147} \hat{n} \cdot \vec{v}_1 \vec{S}_1 \cdot \vec{v}_2 \hat{n} \cdot \vec{S}_1 - \frac{732}{49} \hat{n} \cdot \vec{v}_2 \vec{S}_1 \cdot \vec{v}_2 \hat{n} \cdot \vec{S}_1 + \frac{1137 \left( \vec{S}_1 \cdot \vec{v}_2 \right)^2}{1225} - \\
& \quad \left. \frac{723}{98} \left( \hat{n} \cdot \vec{v}_2 \right)^2 \vec{S}_1 \cdot \vec{S}_1 + \frac{1385}{294} \hat{n} \cdot \vec{v}_1 \hat{n} \cdot \vec{v}_2 \vec{S}_1 \cdot \vec{S}_1 - \frac{109}{147} \vec{S}_1 \cdot \vec{v}_1 \vec{S}_1 \cdot \vec{v}_2 - \frac{55}{98} \vec{S}_1 \cdot \vec{S}_1 \vec{v}_1 \cdot \vec{v}_2 + \frac{3237 \vec{S}_1 \cdot \vec{S}_1 \vec{v}_2 \cdot \vec{v}_2}{2450} \right) + \\
& \left( \frac{1}{r^4} \left( -\frac{27}{7} \hat{n} \cdot \vec{a}_2 \left( \hat{n} \cdot \vec{S}_1 \right)^2 - \frac{54}{7} \hat{n} \cdot \vec{S}_1 \hat{n} \cdot \vec{v}_2 \hat{n} \cdot \vec{S}_1 + \frac{54}{35} \vec{S}_1 \cdot \vec{v}_2 \hat{n} \cdot \vec{S}_1 + \frac{54}{35} \vec{S}_1 \cdot \vec{a}_2 \hat{n} \cdot \vec{S}_1 + \right. \right. \\
& \quad \left. \frac{54}{35} \hat{n} \cdot \vec{v}_2 \vec{S}_1 \cdot \vec{S}_1 + \frac{27}{35} \hat{n} \cdot \vec{a}_2 \vec{S}_1 \cdot \vec{S}_1 + \frac{54}{35} \hat{n} \cdot \vec{S}_1 \vec{S}_1 \cdot \vec{v}_2 \right) + \frac{1}{r^5} \\
& \quad \left( -27 \left( \hat{n} \cdot \vec{v}_2 \right)^2 \left( \hat{n} \cdot \vec{S}_1 \right)^2 + 20 \hat{n} \cdot \vec{v}_1 \hat{n} \cdot \vec{v}_2 \left( \hat{n} \cdot \vec{S}_1 \right)^2 - \frac{20}{7} \vec{v}_1 \cdot \vec{v}_2 \left( \hat{n} \cdot \vec{S}_1 \right)^2 + \frac{27}{7} \vec{v}_2 \cdot \vec{v}_2 \left( \hat{n} \cdot \vec{S}_1 \right)^2 - \right. \\
& \quad \frac{40}{7} \hat{n} \cdot \vec{v}_2 \vec{S}_1 \cdot \vec{v}_1 \hat{n} \cdot \vec{S}_1 - \frac{40}{7} \hat{n} \cdot \vec{v}_1 \vec{S}_1 \cdot \vec{v}_2 \hat{n} \cdot \vec{S}_1 + \frac{108}{7} \hat{n} \cdot \vec{v}_2 \vec{S}_1 \cdot \vec{v}_2 \hat{n} \cdot \vec{S}_1 - \frac{54}{35} \left( \vec{S}_1 \cdot \vec{v}_2 \right)^2 + \\
& \quad \left. \frac{27}{7} \left( \hat{n} \cdot \vec{v}_2 \right)^2 \vec{S}_1 \cdot \vec{S}_1 - \frac{20}{7} \hat{n} \cdot \vec{v}_1 \hat{n} \cdot \vec{v}_2 \vec{S}_1 \cdot \vec{S}_1 + \frac{8}{7} \vec{S}_1 \cdot \vec{v}_1 \vec{S}_1 \cdot \vec{v}_2 + \frac{4}{7} \vec{S}_1 \cdot \vec{S}_1 \vec{v}_1 \cdot \vec{v}_2 - \frac{27}{35} \vec{S}_1 \cdot \vec{S}_1 \vec{v}_2 \cdot \vec{v}_2 \right) \Bigg) \\
& \log \left( \frac{r}{R_0} \right) + \frac{1}{\epsilon_d} \left( \frac{1}{r^4} \left( \frac{9}{7} \hat{n} \cdot \vec{a}_2 \left( \hat{n} \cdot \vec{S}_1 \right)^2 + \frac{18}{7} \hat{n} \cdot \vec{S}_1 \hat{n} \cdot \vec{v}_2 \hat{n} \cdot \vec{S}_1 - \frac{18}{35} \vec{S}_1 \cdot \vec{v}_2 \hat{n} \cdot \vec{S}_1 - \frac{18}{35} \vec{S}_1 \cdot \vec{a}_2 \hat{n} \cdot \vec{S}_1 - \right. \right. \\
& \quad \left. \frac{18}{35} \hat{n} \cdot \vec{v}_2 \vec{S}_1 \cdot \vec{S}_1 - \frac{9}{35} \hat{n} \cdot \vec{a}_2 \vec{S}_1 \cdot \vec{S}_1 - \frac{18}{35} \hat{n} \cdot \vec{S}_1 \vec{S}_1 \cdot \vec{v}_2 \right) + \frac{1}{r^5} \\
& \quad \left( 9 \left( \hat{n} \cdot \vec{v}_2 \right)^2 \left( \hat{n} \cdot \vec{S}_1 \right)^2 - \frac{20}{3} \hat{n} \cdot \vec{v}_1 \hat{n} \cdot \vec{v}_2 \left( \hat{n} \cdot \vec{S}_1 \right)^2 + \frac{20}{21} \vec{v}_1 \cdot \vec{v}_2 \left( \hat{n} \cdot \vec{S}_1 \right)^2 - \frac{9}{7} \vec{v}_2 \cdot \vec{v}_2 \left( \hat{n} \cdot \vec{S}_1 \right)^2 + \right. \\
& \quad \frac{40}{21} \hat{n} \cdot \vec{v}_2 \vec{S}_1 \cdot \vec{v}_1 \hat{n} \cdot \vec{S}_1 + \frac{40}{21} \hat{n} \cdot \vec{v}_1 \vec{S}_1 \cdot \vec{v}_2 \hat{n} \cdot \vec{S}_1 - \frac{36}{7} \hat{n} \cdot \vec{v}_2 \vec{S}_1 \cdot \vec{v}_2 \hat{n} \cdot \vec{S}_1 + \frac{18}{35} \left( \vec{S}_1 \cdot \vec{v}_2 \right)^2 - \frac{9}{7} \left( \hat{n} \cdot \vec{v}_2 \right)^2 \vec{S}_1 \cdot \vec{S}_1 + \\
& \quad \left. \frac{20}{21} \hat{n} \cdot \vec{v}_1 \hat{n} \cdot \vec{v}_2 \vec{S}_1 \cdot \vec{S}_1 - \frac{8}{21} \vec{S}_1 \cdot \vec{v}_1 \vec{S}_1 \cdot \vec{v}_2 - \frac{4}{21} \vec{S}_1 \cdot \vec{S}_1 \vec{v}_1 \cdot \vec{v}_2 + \frac{9}{35} \vec{S}_1 \cdot \vec{S}_1 \vec{v}_2 \cdot \vec{v}_2 \right) \Bigg) \Bigg\} C_{ES^2_1} \}
\end{aligned}$$

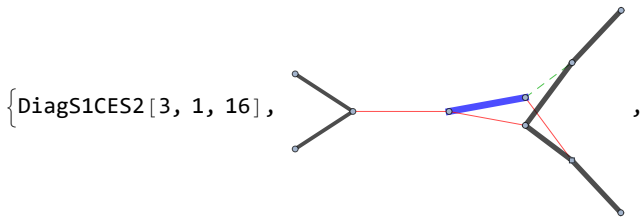

$$\begin{aligned}
& G^3 m_1 m_2 \left( \frac{1}{r^4} \left( -9 \hat{n} \cdot \vec{a}_1 \left( \hat{n} \cdot \vec{S}_1 \right)^2 - 6 \hat{n} \cdot \vec{S}_1 \hat{n} \cdot \vec{v}_1 \hat{n} \cdot \vec{S}_1 + \frac{38}{25} \vec{S}_1 \cdot \vec{v}_1 \hat{n} \cdot \vec{S}_1 + \frac{38}{25} \vec{S}_1 \cdot \vec{a}_1 \hat{n} \cdot \vec{S}_1 + \frac{38}{25} \hat{n} \cdot \vec{v}_1 \vec{S}_1 \cdot \vec{S}_1 + \right. \right. \\
& \quad \frac{69}{25} \hat{n} \cdot \vec{a}_1 \vec{S}_1 \cdot \vec{S}_1 + \frac{38}{25} \hat{n} \cdot \vec{S}_1 \vec{S}_1 \cdot \vec{v}_1 \Bigg) + \frac{1}{r^5} \left( 20 \left( \hat{n} \cdot \vec{v}_1 \right)^2 \left( \hat{n} \cdot \vec{S}_1 \right)^2 - \frac{88}{49} \vec{v}_1 \cdot \vec{v}_1 \left( \hat{n} \cdot \vec{S}_1 \right)^2 - \right. \\
& \quad \left. \frac{660}{49} \hat{n} \cdot \vec{v}_1 \vec{S}_1 \cdot \vec{v}_1 \hat{n} \cdot \vec{S}_1 + \frac{1524 \left( \vec{S}_1 \cdot \vec{v}_1 \right)^2}{1225} - \frac{144}{49} \left( \hat{n} \cdot \vec{v}_1 \right)^2 \vec{S}_1 \cdot \vec{S}_1 + \frac{412 \vec{S}_1 \cdot \vec{S}_1 \vec{v}_1 \cdot \vec{v}_1}{1225} \right) +
\end{aligned}$$

$$\begin{aligned}
& \left( \frac{1}{r^4} \left( 6 \hat{n} \cdot \vec{a}_1 (\hat{n} \cdot \vec{S}_1)^2 + 12 \hat{n} \cdot \vec{S}_1 \hat{n} \cdot \vec{v}_1 \hat{n} \cdot \vec{S}_1 - \frac{12}{5} \vec{S}_1 \cdot \vec{v}_1 \hat{n} \cdot \vec{S}_1 - \frac{12}{5} \vec{S}_1 \cdot \vec{a}_1 \hat{n} \cdot \vec{S}_1 - \frac{12}{5} \hat{n} \cdot \vec{v}_1 \vec{S}_1 \cdot \vec{S}_1 - \right. \right. \\
& \quad \frac{6}{5} \hat{n} \cdot \vec{a}_1 \vec{S}_1 \cdot \vec{S}_1 - \frac{12}{5} \hat{n} \cdot \vec{S}_1 \vec{S}_1 \cdot \vec{v}_1 \left. \right) + \frac{1}{r^5} \left( -24 (\hat{n} \cdot \vec{v}_1)^2 (\hat{n} \cdot \vec{S}_1)^2 + \frac{24}{7} \vec{v}_1 \cdot \vec{v}_1 (\hat{n} \cdot \vec{S}_1)^2 + \right. \\
& \quad \frac{96}{7} \hat{n} \cdot \vec{v}_1 \vec{S}_1 \cdot \vec{v}_1 \hat{n} \cdot \vec{S}_1 - \frac{48}{35} (\vec{S}_1 \cdot \vec{v}_1)^2 + \frac{24}{7} (\hat{n} \cdot \vec{v}_1)^2 \vec{S}_1 \cdot \vec{S}_1 - \frac{24}{35} \vec{S}_1 \cdot \vec{S}_1 \vec{v}_1 \cdot \vec{v}_1 \left. \right) \log \left( \frac{r}{R_\theta} \right) + \\
& \quad \frac{1}{\epsilon_d} \left( \frac{1}{r^4} \left( -2 \hat{n} \cdot \vec{a}_1 (\hat{n} \cdot \vec{S}_1)^2 - 4 \hat{n} \cdot \vec{S}_1 \hat{n} \cdot \vec{v}_1 \hat{n} \cdot \vec{S}_1 + \frac{4}{5} \vec{S}_1 \cdot \vec{v}_1 \hat{n} \cdot \vec{S}_1 + \frac{4}{5} \vec{S}_1 \cdot \vec{a}_1 \hat{n} \cdot \vec{S}_1 + \frac{4}{5} \hat{n} \cdot \vec{v}_1 \vec{S}_1 \cdot \vec{S}_1 + \right. \right. \\
& \quad \frac{2}{5} \hat{n} \cdot \vec{a}_1 \vec{S}_1 \cdot \vec{S}_1 + \frac{4}{5} \hat{n} \cdot \vec{S}_1 \vec{S}_1 \cdot \vec{v}_1 \left. \right) + \frac{1}{r^5} \left( 8 (\hat{n} \cdot \vec{v}_1)^2 (\hat{n} \cdot \vec{S}_1)^2 - \frac{8}{7} \vec{v}_1 \cdot \vec{v}_1 (\hat{n} \cdot \vec{S}_1)^2 - \right. \\
& \quad \left. \left. \frac{32}{7} \hat{n} \cdot \vec{v}_1 \vec{S}_1 \cdot \vec{v}_1 \hat{n} \cdot \vec{S}_1 + \frac{16}{35} (\vec{S}_1 \cdot \vec{v}_1)^2 - \frac{8}{7} (\hat{n} \cdot \vec{v}_1)^2 \vec{S}_1 \cdot \vec{S}_1 + \frac{8}{35} \vec{S}_1 \cdot \vec{S}_1 \vec{v}_1 \cdot \vec{v}_1 \right) \right) \Bigg\} c_{ES^2_1} \}
\end{aligned}$$

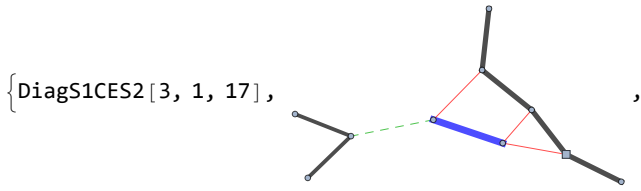

$$\begin{aligned}
& G^3 m_1 m_2 \left( \frac{\frac{299}{49} \hat{n} \cdot \vec{a}_2 (\hat{n} \cdot \vec{S}_1)^2 - \frac{114}{49} \vec{S}_1 \cdot \vec{a}_2 \hat{n} \cdot \vec{S}_1 - \frac{71}{49} \hat{n} \cdot \vec{a}_2 \vec{S}_1 \cdot \vec{S}_1}{r^4} + \frac{1}{r^5} \right. \\
& \quad \left( 47 (\hat{n} \cdot \vec{v}_2)^2 (\hat{n} \cdot \vec{S}_1)^2 - \frac{33}{4} \hat{n} \cdot \vec{v}_1 \hat{n} \cdot \vec{v}_2 (\hat{n} \cdot \vec{S}_1)^2 + \frac{577}{588} \vec{v}_1 \cdot \vec{v}_2 (\hat{n} \cdot \vec{S}_1)^2 - \frac{299}{49} \vec{v}_2 \cdot \vec{v}_2 (\hat{n} \cdot \vec{S}_1)^2 + \right. \\
& \quad \frac{241}{294} \hat{n} \cdot \vec{v}_2 \vec{S}_1 \cdot \vec{v}_1 \hat{n} \cdot \vec{S}_1 + \frac{745}{294} \hat{n} \cdot \vec{v}_1 \vec{S}_1 \cdot \vec{v}_2 \hat{n} \cdot \vec{S}_1 - \frac{1252}{49} \hat{n} \cdot \vec{v}_2 \vec{S}_1 \cdot \vec{v}_2 \hat{n} \cdot \vec{S}_1 + \frac{114}{49} (\vec{S}_1 \cdot \vec{v}_2)^2 - \\
& \quad \frac{397}{49} (\hat{n} \cdot \vec{v}_2)^2 \vec{S}_1 \cdot \vec{S}_1 + \frac{351}{196} \hat{n} \cdot \vec{v}_1 \hat{n} \cdot \vec{v}_2 \vec{S}_1 \cdot \vec{S}_1 - \frac{3}{98} \vec{S}_1 \cdot \vec{v}_1 \vec{S}_1 \cdot \vec{v}_2 - \frac{205}{588} \vec{S}_1 \cdot \vec{S}_1 \vec{v}_1 \cdot \vec{v}_2 + \frac{71}{49} \vec{S}_1 \cdot \vec{S}_1 \vec{v}_2 \cdot \vec{v}_2 \left. \right) + \\
& \quad \left( \frac{-\frac{30}{7} \hat{n} \cdot \vec{a}_2 (\hat{n} \cdot \vec{S}_1)^2 + \frac{12}{7} \vec{S}_1 \cdot \vec{a}_2 \hat{n} \cdot \vec{S}_1 + \frac{6}{7} \hat{n} \cdot \vec{a}_2 \vec{S}_1 \cdot \vec{S}_1}{r^4} + \frac{1}{r^5} \right. \\
& \quad \left( -30 (\hat{n} \cdot \vec{v}_2)^2 (\hat{n} \cdot \vec{S}_1)^2 + 5 \hat{n} \cdot \vec{v}_1 \hat{n} \cdot \vec{v}_2 (\hat{n} \cdot \vec{S}_1)^2 - \frac{5}{7} \vec{v}_1 \cdot \vec{v}_2 (\hat{n} \cdot \vec{S}_1)^2 + \frac{30}{7} \vec{v}_2 \cdot \vec{v}_2 (\hat{n} \cdot \vec{S}_1)^2 - \right. \\
& \quad \frac{10}{7} \hat{n} \cdot \vec{v}_2 \vec{S}_1 \cdot \vec{v}_1 \hat{n} \cdot \vec{S}_1 - \frac{10}{7} \hat{n} \cdot \vec{v}_1 \vec{S}_1 \cdot \vec{v}_2 \hat{n} \cdot \vec{S}_1 + \frac{120}{7} \hat{n} \cdot \vec{v}_2 \vec{S}_1 \cdot \vec{v}_2 \hat{n} \cdot \vec{S}_1 - \frac{12}{7} (\vec{S}_1 \cdot \vec{v}_2)^2 + \\
& \quad \left. \left. \frac{30}{7} (\hat{n} \cdot \vec{v}_2)^2 \vec{S}_1 \cdot \vec{S}_1 - \frac{5}{7} \hat{n} \cdot \vec{v}_1 \hat{n} \cdot \vec{v}_2 \vec{S}_1 \cdot \vec{S}_1 + \frac{2}{7} \vec{S}_1 \cdot \vec{v}_1 \vec{S}_1 \cdot \vec{v}_2 + \frac{1}{7} \vec{S}_1 \cdot \vec{S}_1 \vec{v}_1 \cdot \vec{v}_2 - \frac{6}{7} \vec{S}_1 \cdot \vec{S}_1 \vec{v}_2 \cdot \vec{v}_2 \right) \right) \\
& \quad \log \left( \frac{r}{R_\theta} \right) + \frac{1}{\epsilon_d} \left( \frac{\frac{10}{7} \hat{n} \cdot \vec{a}_2 (\hat{n} \cdot \vec{S}_1)^2 - \frac{4}{7} \vec{S}_1 \cdot \vec{a}_2 \hat{n} \cdot \vec{S}_1 - \frac{2}{7} \hat{n} \cdot \vec{a}_2 \vec{S}_1 \cdot \vec{S}_1}{r^4} + \frac{1}{r^5} \right. \\
& \quad \left( 10 (\hat{n} \cdot \vec{v}_2)^2 (\hat{n} \cdot \vec{S}_1)^2 - \frac{5}{3} \hat{n} \cdot \vec{v}_1 \hat{n} \cdot \vec{v}_2 (\hat{n} \cdot \vec{S}_1)^2 + \frac{5}{21} \vec{v}_1 \cdot \vec{v}_2 (\hat{n} \cdot \vec{S}_1)^2 - \frac{10}{7} \vec{v}_2 \cdot \vec{v}_2 (\hat{n} \cdot \vec{S}_1)^2 + \right. \\
& \quad \frac{10}{21} \hat{n} \cdot \vec{v}_2 \vec{S}_1 \cdot \vec{v}_1 \hat{n} \cdot \vec{S}_1 + \frac{10}{21} \hat{n} \cdot \vec{v}_1 \vec{S}_1 \cdot \vec{v}_2 \hat{n} \cdot \vec{S}_1 - \frac{40}{7} \hat{n} \cdot \vec{v}_2 \vec{S}_1 \cdot \vec{v}_2 \hat{n} \cdot \vec{S}_1 + \frac{4}{7} (\vec{S}_1 \cdot \vec{v}_2)^2 - \frac{10}{7} (\hat{n} \cdot \vec{v}_2)^2 \vec{S}_1 \cdot \vec{S}_1 + \\
& \quad \left. \left. \frac{5}{21} \hat{n} \cdot \vec{v}_1 \hat{n} \cdot \vec{v}_2 \vec{S}_1 \cdot \vec{S}_1 - \frac{2}{21} \vec{S}_1 \cdot \vec{v}_1 \vec{S}_1 \cdot \vec{v}_2 - \frac{1}{21} \vec{S}_1 \cdot \vec{S}_1 \vec{v}_1 \cdot \vec{v}_2 + \frac{2}{7} \vec{S}_1 \cdot \vec{S}_1 \vec{v}_2 \cdot \vec{v}_2 \right) \right) \Bigg\} c_{ES^2_1} \}
\end{aligned}$$

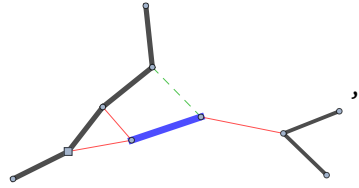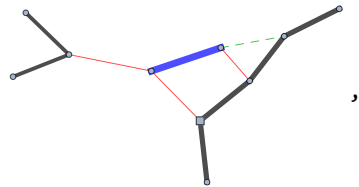

$$G^3 m_1 m_2 C_{\text{ES}^2 1} \left( \frac{-30 \hat{n} \cdot \vec{a}_1 \left( \hat{n} \cdot \vec{S}_1 \right)^2 + 12 \vec{S}_1 \cdot \vec{a}_1 \hat{n} \cdot \vec{S}_1 + 6 \vec{S}_1 \cdot \vec{S}_1 \hat{n} \cdot \vec{a}_1}{r^4 \in_d} + \frac{\log \left( \frac{r}{R_\theta} \right) \left( 90 \hat{n} \cdot \vec{a}_1 \left( \hat{n} \cdot \vec{S}_1 \right)^2 - 36 \vec{S}_1 \cdot \vec{a}_1 \hat{n} \cdot \vec{S}_1 - 18 \vec{S}_1 \cdot \vec{S}_1 \hat{n} \cdot \vec{a}_1 \right)}{r^4} + \frac{-91 \hat{n} \cdot \vec{a}_1 \left( \hat{n} \cdot \vec{S}_1 \right)^2 + 34 \vec{S}_1 \cdot \vec{a}_1 \hat{n} \cdot \vec{S}_1 + 23 \vec{S}_1 \cdot \vec{S}_1 \hat{n} \cdot \vec{a}_1}{r^4} \right) \Bigg\}$$

{DiagS1CES2[3, 1, 20],

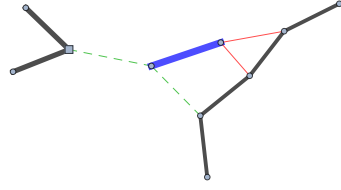

,  $\frac{1}{m_1}$

$$G^3 m_2^3 \left( \frac{-20 \hat{n} \cdot \vec{S}_1 \hat{n} \cdot \vec{S}_1 \hat{n} \cdot \vec{v}_2 + \frac{168}{25} \vec{S}_1 \cdot \vec{S}_1 \hat{n} \cdot \vec{v}_2 + \frac{78}{25} \hat{n} \cdot \vec{S}_1 \vec{S}_1 \cdot \vec{v}_2 + \frac{78}{25} \hat{n} \cdot \vec{S}_1 \vec{S}_1 \cdot \vec{v}_2}{r^4} + \right. \\ \left. \frac{1}{r^5} \left( 76 \hat{n} \cdot \vec{v}_1 \hat{n} \cdot \vec{v}_2 (\hat{n} \cdot \vec{S}_1)^2 - 8 \vec{v}_1 \cdot \vec{v}_2 (\hat{n} \cdot \vec{S}_1)^2 - 20 \hat{n} \cdot \vec{v}_2 \vec{S}_1 \cdot \vec{v}_1 \hat{n} \cdot \vec{S}_1 - \right. \right. \\ \left. \left. 20 \hat{n} \cdot \vec{v}_1 \vec{S}_1 \cdot \vec{v}_2 \hat{n} \cdot \vec{S}_1 - 16 \hat{n} \cdot \vec{v}_1 \hat{n} \cdot \vec{v}_2 \vec{S}_1 \cdot \vec{S}_1 + \frac{88}{25} \vec{S}_1 \cdot \vec{v}_1 \vec{S}_1 \cdot \vec{v}_2 + \frac{44}{25} \vec{S}_1 \cdot \vec{S}_1 \vec{v}_1 \cdot \vec{v}_2 \right) + \right. \\ \left. \left( \frac{12 \hat{n} \cdot \vec{S}_1 \hat{n} \cdot \vec{S}_1 \hat{n} \cdot \vec{v}_2 - \frac{12}{5} \vec{S}_1 \cdot \vec{S}_1 \hat{n} \cdot \vec{v}_2 - \frac{12}{5} \hat{n} \cdot \vec{S}_1 \vec{S}_1 \cdot \vec{v}_2 - \frac{12}{5} \hat{n} \cdot \vec{S}_1 \vec{S}_1 \cdot \vec{v}_2}{r^4} + \frac{1}{r^5} \right. \right. \\ \left. \left. \left( -42 \hat{n} \cdot \vec{v}_1 \hat{n} \cdot \vec{v}_2 (\hat{n} \cdot \vec{S}_1)^2 + 6 \vec{v}_1 \cdot \vec{v}_2 (\hat{n} \cdot \vec{S}_1)^2 + 12 \hat{n} \cdot \vec{v}_2 \vec{S}_1 \cdot \vec{v}_1 \hat{n} \cdot \vec{S}_1 + 12 \hat{n} \cdot \vec{v}_1 \vec{S}_1 \cdot \vec{v}_2 \hat{n} \cdot \vec{S}_1 + \right. \right. \right. \\ \left. \left. \left. 6 \hat{n} \cdot \vec{v}_1 \hat{n} \cdot \vec{v}_2 \vec{S}_1 \cdot \vec{S}_1 - \frac{12}{5} \vec{S}_1 \cdot \vec{v}_1 \vec{S}_1 \cdot \vec{v}_2 - \frac{6}{5} \vec{S}_1 \cdot \vec{S}_1 \vec{v}_1 \cdot \vec{v}_2 \right) \log\left(\frac{r}{R_0}\right) + \right. \right. \\ \left. \left. \frac{1}{\epsilon_d} \left( \frac{-4 \hat{n} \cdot \vec{S}_1 \hat{n} \cdot \vec{S}_1 \hat{n} \cdot \vec{v}_2 + \frac{4}{5} \vec{S}_1 \cdot \vec{S}_1 \hat{n} \cdot \vec{v}_2 + \frac{4}{5} \hat{n} \cdot \vec{S}_1 \vec{S}_1 \cdot \vec{v}_2 + \frac{4}{5} \hat{n} \cdot \vec{S}_1 \vec{S}_1 \cdot \vec{v}_2}{r^4} + \frac{1}{r^5} \right. \right. \right. \\ \left. \left. \left( 14 \hat{n} \cdot \vec{v}_1 \hat{n} \cdot \vec{v}_2 (\hat{n} \cdot \vec{S}_1)^2 - 2 \vec{v}_1 \cdot \vec{v}_2 (\hat{n} \cdot \vec{S}_1)^2 - 4 \hat{n} \cdot \vec{v}_2 \vec{S}_1 \cdot \vec{v}_1 \hat{n} \cdot \vec{S}_1 - \right. \right. \right. \\ \left. \left. \left. 4 \hat{n} \cdot \vec{v}_1 \vec{S}_1 \cdot \vec{v}_2 \hat{n} \cdot \vec{S}_1 - 2 \hat{n} \cdot \vec{v}_1 \hat{n} \cdot \vec{v}_2 \vec{S}_1 \cdot \vec{S}_1 + \frac{4}{5} \vec{S}_1 \cdot \vec{v}_1 \vec{S}_1 \cdot \vec{v}_2 + \frac{2}{5} \vec{S}_1 \cdot \vec{S}_1 \vec{v}_1 \cdot \vec{v}_2 \right) \right) \right) \Bigg\} C_{ES^2 1}$$

{DiagS1CES2[3, 1, 21],

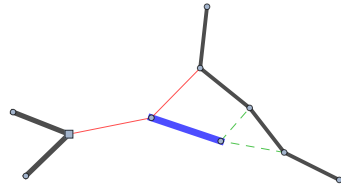

,  $\frac{1}{m_1}$

$$G^3 m_2^3 C_{ES^2 1} \left( \frac{1}{r^5 \epsilon_d} \left( -70 (\hat{n} \cdot \vec{S}_1)^2 (\hat{n} \cdot \vec{v}_2)^2 + 10 \vec{v}_2 \cdot \vec{v}_2 (\hat{n} \cdot \vec{S}_1)^2 + 40 \hat{n} \cdot \vec{S}_1 \hat{n} \cdot \vec{v}_2 \vec{S}_1 \cdot \vec{v}_2 + 10 \vec{S}_1 \cdot \vec{S}_1 (\hat{n} \cdot \vec{v}_2)^2 - \right. \right. \\ \left. \left. 4 (\vec{S}_1 \cdot \vec{v}_2)^2 - 2 \vec{S}_1 \cdot \vec{S}_1 \vec{v}_2 \cdot \vec{v}_2 \right) + \frac{1}{r^5} \log\left(\frac{r}{R_0}\right) \left( 210 (\hat{n} \cdot \vec{S}_1)^2 (\hat{n} \cdot \vec{v}_2)^2 - 30 \vec{v}_2 \cdot \vec{v}_2 (\hat{n} \cdot \vec{S}_1)^2 - \right. \right. \\ \left. \left. 120 \hat{n} \cdot \vec{S}_1 \hat{n} \cdot \vec{v}_2 \vec{S}_1 \cdot \vec{v}_2 - 30 \vec{S}_1 \cdot \vec{S}_1 (\hat{n} \cdot \vec{v}_2)^2 + 12 (\vec{S}_1 \cdot \vec{v}_2)^2 + 6 \vec{S}_1 \cdot \vec{S}_1 \vec{v}_2 \cdot \vec{v}_2 \right) + \frac{1}{r^5} \left( -177 (\hat{n} \cdot \vec{S}_1)^2 (\hat{n} \cdot \vec{v}_2)^2 + \right. \right. \\ \left. \left. 31 \vec{v}_2 \cdot \vec{v}_2 (\hat{n} \cdot \vec{S}_1)^2 + 84 \hat{n} \cdot \vec{S}_1 \hat{n} \cdot \vec{v}_2 \vec{S}_1 \cdot \vec{v}_2 + 51 \vec{S}_1 \cdot \vec{S}_1 (\hat{n} \cdot \vec{v}_2)^2 - 6 (\vec{S}_1 \cdot \vec{v}_2)^2 - 15 \vec{S}_1 \cdot \vec{S}_1 \vec{v}_2 \cdot \vec{v}_2 \right) \right) \Bigg\}$$



{DiagS1CES2[3, 1, 22],

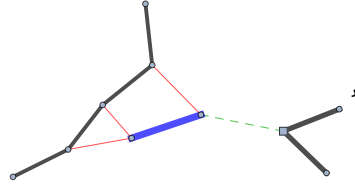

$$\begin{aligned}
 & \frac{1}{m_1} G^3 m_2^3 \left( \frac{7 \left( \hat{n} \cdot \vec{S}_1 \right)^2 + 7 \hat{n} \cdot \vec{S}_1 \hat{n} \cdot \vec{S}_1 - \frac{11}{3} \vec{S}_1 \cdot \vec{S}_1 - \frac{11}{3} \vec{S}_1 \cdot \vec{S}_1}{r^3} + \frac{1}{r^4} \right. \\
 & \left( -\frac{41}{2} \hat{n} \cdot \vec{a}_1 \left( \hat{n} \cdot \vec{S}_1 \right)^2 - 82 \hat{n} \cdot \vec{S}_1 \hat{n} \cdot \vec{v}_1 \hat{n} \cdot \vec{S}_1 + 15 \hat{n} \cdot \vec{S}_1 \hat{n} \cdot \vec{v}_2 \hat{n} \cdot \vec{S}_1 + 14 \vec{S}_1 \cdot \vec{v}_1 \hat{n} \cdot \vec{S}_1 - \frac{53}{25} \vec{S}_1 \cdot \vec{v}_2 \hat{n} \cdot \vec{S}_1 + \right. \\
 & \left. 7 \vec{S}_1 \cdot \vec{a}_1 \hat{n} \cdot \vec{S}_1 + 26 \hat{n} \cdot \vec{v}_1 \vec{S}_1 \cdot \vec{S}_1 - \frac{143}{25} \hat{n} \cdot \vec{v}_2 \vec{S}_1 \cdot \vec{S}_1 + \frac{13}{2} \hat{n} \cdot \vec{a}_1 \vec{S}_1 \cdot \vec{S}_1 + 14 \hat{n} \cdot \vec{S}_1 \vec{S}_1 \cdot \vec{v}_1 - \frac{53}{25} \hat{n} \cdot \vec{S}_1 \vec{S}_1 \cdot \vec{v}_2 \right) + \\
 & \frac{1}{r^5} \left( \frac{317}{2} \left( \hat{n} \cdot \vec{v}_1 \right)^2 \left( \hat{n} \cdot \vec{S}_1 \right)^2 - \frac{117}{2} \hat{n} \cdot \vec{v}_1 \hat{n} \cdot \vec{v}_2 \left( \hat{n} \cdot \vec{S}_1 \right)^2 - \frac{41}{2} \vec{v}_1 \cdot \vec{v}_1 \left( \hat{n} \cdot \vec{S}_1 \right)^2 + \frac{11}{2} \vec{v}_1 \cdot \vec{v}_2 \left( \hat{n} \cdot \vec{S}_1 \right)^2 - \right. \\
 & \left. 82 \hat{n} \cdot \vec{v}_1 \vec{S}_1 \cdot \vec{v}_1 \hat{n} \cdot \vec{S}_1 + 15 \hat{n} \cdot \vec{v}_2 \vec{S}_1 \cdot \vec{v}_1 \hat{n} \cdot \vec{S}_1 + 15 \hat{n} \cdot \vec{v}_1 \vec{S}_1 \cdot \vec{v}_2 \hat{n} \cdot \vec{S}_1 + 7 \left( \vec{S}_1 \cdot \vec{v}_1 \right)^2 - \right. \\
 & \left. \frac{71}{2} \left( \hat{n} \cdot \vec{v}_1 \right)^2 \vec{S}_1 \cdot \vec{S}_1 + \frac{27}{2} \hat{n} \cdot \vec{v}_1 \hat{n} \cdot \vec{v}_2 \vec{S}_1 \cdot \vec{S}_1 - \frac{63}{25} \vec{S}_1 \cdot \vec{v}_1 \vec{S}_1 \cdot \vec{v}_2 + \frac{13}{2} \vec{S}_1 \cdot \vec{S}_1 \vec{v}_1 \cdot \vec{v}_1 - \frac{63}{50} \vec{S}_1 \cdot \vec{S}_1 \vec{v}_1 \cdot \vec{v}_2 \right) + \\
 & \left( \frac{-6 \left( \hat{n} \cdot \vec{S}_1 \right)^2 - 6 \hat{n} \cdot \vec{S}_1 \hat{n} \cdot \vec{S}_1 + 2 \vec{S}_1 \cdot \vec{S}_1 + 2 \vec{S}_1 \cdot \vec{S}_1}{r^3} + \frac{1}{r^4} \right. \\
 & \left( 15 \hat{n} \cdot \vec{a}_1 \left( \hat{n} \cdot \vec{S}_1 \right)^2 + 60 \hat{n} \cdot \vec{S}_1 \hat{n} \cdot \vec{v}_1 \hat{n} \cdot \vec{S}_1 - 12 \hat{n} \cdot \vec{S}_1 \hat{n} \cdot \vec{v}_2 \hat{n} \cdot \vec{S}_1 - 12 \vec{S}_1 \cdot \vec{v}_1 \hat{n} \cdot \vec{S}_1 + \frac{12}{5} \vec{S}_1 \cdot \vec{v}_2 \hat{n} \cdot \vec{S}_1 - \right. \\
 & \left. 6 \vec{S}_1 \cdot \vec{a}_1 \hat{n} \cdot \vec{S}_1 - 12 \hat{n} \cdot \vec{v}_1 \vec{S}_1 \cdot \vec{S}_1 + \frac{12}{5} \hat{n} \cdot \vec{v}_2 \vec{S}_1 \cdot \vec{S}_1 - 3 \hat{n} \cdot \vec{a}_1 \vec{S}_1 \cdot \vec{S}_1 - 12 \hat{n} \cdot \vec{S}_1 \vec{S}_1 \cdot \vec{v}_1 + \frac{12}{5} \hat{n} \cdot \vec{S}_1 \vec{S}_1 \cdot \vec{v}_2 \right) + \\
 & \frac{1}{r^5} \left( -105 \left( \hat{n} \cdot \vec{v}_1 \right)^2 \left( \hat{n} \cdot \vec{S}_1 \right)^2 + 42 \hat{n} \cdot \vec{v}_1 \hat{n} \cdot \vec{v}_2 \left( \hat{n} \cdot \vec{S}_1 \right)^2 + 15 \vec{v}_1 \cdot \vec{v}_1 \left( \hat{n} \cdot \vec{S}_1 \right)^2 - 6 \vec{v}_1 \cdot \vec{v}_2 \left( \hat{n} \cdot \vec{S}_1 \right)^2 + \right. \\
 & \left. 60 \hat{n} \cdot \vec{v}_1 \vec{S}_1 \cdot \vec{v}_1 \hat{n} \cdot \vec{S}_1 - 12 \hat{n} \cdot \vec{v}_2 \vec{S}_1 \cdot \vec{v}_1 \hat{n} \cdot \vec{S}_1 - 12 \hat{n} \cdot \vec{v}_1 \vec{S}_1 \cdot \vec{v}_2 \hat{n} \cdot \vec{S}_1 - 6 \left( \vec{S}_1 \cdot \vec{v}_1 \right)^2 + \right. \\
 & \left. 15 \left( \hat{n} \cdot \vec{v}_1 \right)^2 \vec{S}_1 \cdot \vec{S}_1 - 6 \hat{n} \cdot \vec{v}_1 \hat{n} \cdot \vec{v}_2 \vec{S}_1 \cdot \vec{S}_1 + \frac{12}{5} \vec{S}_1 \cdot \vec{v}_1 \vec{S}_1 \cdot \vec{v}_2 - 3 \vec{S}_1 \cdot \vec{S}_1 \vec{v}_1 \cdot \vec{v}_1 + \frac{6}{5} \vec{S}_1 \cdot \vec{S}_1 \vec{v}_1 \cdot \vec{v}_2 \right) \left. \right) \\
 & \log \left( \frac{r}{R_\theta} \right) + \frac{1}{\epsilon_d} \left( \frac{2 \left( \hat{n} \cdot \vec{S}_1 \right)^2 + 2 \hat{n} \cdot \vec{S}_1 \hat{n} \cdot \vec{S}_1 - \frac{2}{3} \vec{S}_1 \cdot \vec{S}_1 - \frac{2}{3} \vec{S}_1 \cdot \vec{S}_1}{r^3} + \frac{1}{r^4} \right. \\
 & \left( -5 \hat{n} \cdot \vec{a}_1 \left( \hat{n} \cdot \vec{S}_1 \right)^2 - 20 \hat{n} \cdot \vec{S}_1 \hat{n} \cdot \vec{v}_1 \hat{n} \cdot \vec{S}_1 + 4 \hat{n} \cdot \vec{S}_1 \hat{n} \cdot \vec{v}_2 \hat{n} \cdot \vec{S}_1 + 4 \vec{S}_1 \cdot \vec{v}_1 \hat{n} \cdot \vec{S}_1 - \frac{4}{5} \vec{S}_1 \cdot \vec{v}_2 \hat{n} \cdot \vec{S}_1 + \right. \\
 & \left. 2 \vec{S}_1 \cdot \vec{a}_1 \hat{n} \cdot \vec{S}_1 + 4 \hat{n} \cdot \vec{v}_1 \vec{S}_1 \cdot \vec{S}_1 - \frac{4}{5} \hat{n} \cdot \vec{v}_2 \vec{S}_1 \cdot \vec{S}_1 + \hat{n} \cdot \vec{a}_1 \vec{S}_1 \cdot \vec{S}_1 + 4 \hat{n} \cdot \vec{S}_1 \vec{S}_1 \cdot \vec{v}_1 - \frac{4}{5} \hat{n} \cdot \vec{S}_1 \vec{S}_1 \cdot \vec{v}_2 \right) + \\
 & \frac{1}{r^5} \left( 35 \left( \hat{n} \cdot \vec{v}_1 \right)^2 \left( \hat{n} \cdot \vec{S}_1 \right)^2 - 14 \hat{n} \cdot \vec{v}_1 \hat{n} \cdot \vec{v}_2 \left( \hat{n} \cdot \vec{S}_1 \right)^2 - 5 \vec{v}_1 \cdot \vec{v}_1 \left( \hat{n} \cdot \vec{S}_1 \right)^2 + 2 \vec{v}_1 \cdot \vec{v}_2 \left( \hat{n} \cdot \vec{S}_1 \right)^2 - \right. \\
 & \left. 20 \hat{n} \cdot \vec{v}_1 \vec{S}_1 \cdot \vec{v}_1 \hat{n} \cdot \vec{S}_1 + 4 \hat{n} \cdot \vec{v}_2 \vec{S}_1 \cdot \vec{v}_1 \hat{n} \cdot \vec{S}_1 + 4 \hat{n} \cdot \vec{v}_1 \vec{S}_1 \cdot \vec{v}_2 \hat{n} \cdot \vec{S}_1 + 2 \left( \vec{S}_1 \cdot \vec{v}_1 \right)^2 - 5 \left( \hat{n} \cdot \vec{v}_1 \right)^2 \vec{S}_1 \cdot \vec{S}_1 + \right.
 \end{aligned}$$

$$\left. \left. \left. 2 \hat{n} \cdot \vec{v}_1 \hat{n} \cdot \vec{v}_2 \vec{S}_1 \cdot \vec{S}_1 - \frac{4}{5} \vec{S}_1 \cdot \vec{v}_1 \vec{S}_1 \cdot \vec{v}_2 + \vec{S}_1 \cdot \vec{S}_1 \vec{v}_1 \cdot \vec{v}_1 - \frac{2}{5} \vec{S}_1 \cdot \vec{S}_1 \vec{v}_1 \cdot \vec{v}_2 \right) \right) \right\} C_{ES^2 1} \Bigg\}$$

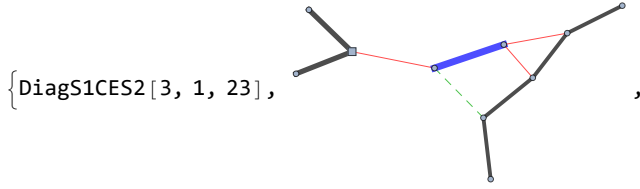

$$\begin{aligned} & \frac{1}{m_1} G^3 m_2^3 \left( \frac{1}{r^4} \left( \frac{41}{2} \hat{n} \cdot \vec{a}_2 (\hat{n} \cdot \vec{S}_1)^2 + 41 \hat{n} \cdot \vec{S}_1 \hat{n} \cdot \vec{v}_2 \hat{n} \cdot \vec{S}_1 - 7 \vec{S}_1 \cdot \vec{v}_2 \hat{n} \cdot \vec{S}_1 - \right. \right. \\ & \quad \left. \left. 7 \vec{S}_1 \cdot \vec{a}_2 \hat{n} \cdot \vec{S}_1 - 13 \hat{n} \cdot \vec{v}_2 \vec{S}_1 \cdot \vec{S}_1 - \frac{13}{2} \hat{n} \cdot \vec{a}_2 \vec{S}_1 \cdot \vec{S}_1 - 7 \hat{n} \cdot \vec{S}_1 \vec{S}_1 \cdot \vec{v}_2 \right) + \frac{1}{r^5} \right. \\ & \quad \left( \frac{117}{2} (\hat{n} \cdot \vec{v}_2)^2 (\hat{n} \cdot \vec{S}_1)^2 - \frac{317}{2} \hat{n} \cdot \vec{v}_1 \hat{n} \cdot \vec{v}_2 (\hat{n} \cdot \vec{S}_1)^2 + \frac{41}{2} \vec{v}_1 \cdot \vec{v}_2 (\hat{n} \cdot \vec{S}_1)^2 - \frac{11}{2} \vec{v}_2 \cdot \vec{v}_2 (\hat{n} \cdot \vec{S}_1)^2 + \right. \\ & \quad \left. 41 \hat{n} \cdot \vec{v}_2 \vec{S}_1 \cdot \vec{v}_1 \hat{n} \cdot \vec{S}_1 + 41 \hat{n} \cdot \vec{v}_1 \vec{S}_1 \cdot \vec{v}_2 \hat{n} \cdot \vec{S}_1 - 30 \hat{n} \cdot \vec{v}_2 \vec{S}_1 \cdot \vec{v}_2 \hat{n} \cdot \vec{S}_1 + \frac{63}{25} (\vec{S}_1 \cdot \vec{v}_2)^2 - \right. \\ & \quad \left. \frac{27}{2} (\hat{n} \cdot \vec{v}_2)^2 \vec{S}_1 \cdot \vec{S}_1 + \frac{71}{2} \hat{n} \cdot \vec{v}_1 \hat{n} \cdot \vec{v}_2 \vec{S}_1 \cdot \vec{S}_1 - 7 \vec{S}_1 \cdot \vec{v}_1 \vec{S}_1 \cdot \vec{v}_2 - \frac{13}{2} \vec{S}_1 \cdot \vec{S}_1 \vec{v}_1 \cdot \vec{v}_2 + \frac{63}{50} \vec{S}_1 \cdot \vec{S}_1 \vec{v}_2 \cdot \vec{v}_2 \right) + \\ & \quad \left( \frac{1}{r^4} \left( -15 \hat{n} \cdot \vec{a}_2 (\hat{n} \cdot \vec{S}_1)^2 - 30 \hat{n} \cdot \vec{S}_1 \hat{n} \cdot \vec{v}_2 \hat{n} \cdot \vec{S}_1 + 6 \vec{S}_1 \cdot \vec{v}_2 \hat{n} \cdot \vec{S}_1 + 6 \vec{S}_1 \cdot \vec{a}_2 \hat{n} \cdot \vec{S}_1 + 6 \hat{n} \cdot \vec{v}_2 \vec{S}_1 \cdot \vec{S}_1 + 3 \hat{n} \cdot \vec{a}_2 \vec{S}_1 \cdot \vec{S}_1 + \right. \right. \\ & \quad \left. \left. 6 \hat{n} \cdot \vec{S}_1 \vec{S}_1 \cdot \vec{v}_2 \right) + \frac{1}{r^5} \left( -42 (\hat{n} \cdot \vec{v}_2)^2 (\hat{n} \cdot \vec{S}_1)^2 + 105 \hat{n} \cdot \vec{v}_1 \hat{n} \cdot \vec{v}_2 (\hat{n} \cdot \vec{S}_1)^2 - 15 \vec{v}_1 \cdot \vec{v}_2 (\hat{n} \cdot \vec{S}_1)^2 + \right. \right. \\ & \quad \left. \left. 6 \vec{v}_2 \cdot \vec{v}_2 (\hat{n} \cdot \vec{S}_1)^2 - 30 \hat{n} \cdot \vec{v}_2 \vec{S}_1 \cdot \vec{v}_1 \hat{n} \cdot \vec{S}_1 - 30 \hat{n} \cdot \vec{v}_1 \vec{S}_1 \cdot \vec{v}_2 \hat{n} \cdot \vec{S}_1 + 24 \hat{n} \cdot \vec{v}_2 \vec{S}_1 \cdot \vec{v}_2 \hat{n} \cdot \vec{S}_1 - \frac{12}{5} (\vec{S}_1 \cdot \vec{v}_2)^2 + \right. \right. \\ & \quad \left. \left. 6 (\hat{n} \cdot \vec{v}_2)^2 \vec{S}_1 \cdot \vec{S}_1 - 15 \hat{n} \cdot \vec{v}_1 \hat{n} \cdot \vec{v}_2 \vec{S}_1 \cdot \vec{S}_1 + 6 \vec{S}_1 \cdot \vec{v}_1 \vec{S}_1 \cdot \vec{v}_2 + 3 \vec{S}_1 \cdot \vec{S}_1 \vec{v}_1 \cdot \vec{v}_2 - \frac{6}{5} \vec{S}_1 \cdot \vec{S}_1 \vec{v}_2 \cdot \vec{v}_2 \right) \right) \log \left( \frac{r}{R_0} \right) + \\ & \quad \frac{1}{\epsilon_d} \left( \frac{1}{r^4} \left( 5 \hat{n} \cdot \vec{a}_2 (\hat{n} \cdot \vec{S}_1)^2 + 10 \hat{n} \cdot \vec{S}_1 \hat{n} \cdot \vec{v}_2 \hat{n} \cdot \vec{S}_1 - 2 \vec{S}_1 \cdot \vec{v}_2 \hat{n} \cdot \vec{S}_1 - 2 \vec{S}_1 \cdot \vec{a}_2 \hat{n} \cdot \vec{S}_1 - 2 \hat{n} \cdot \vec{v}_2 \vec{S}_1 \cdot \vec{S}_1 - \right. \right. \\ & \quad \left. \left. \hat{n} \cdot \vec{a}_2 \vec{S}_1 \cdot \vec{S}_1 - 2 \hat{n} \cdot \vec{S}_1 \vec{S}_1 \cdot \vec{v}_2 \right) + \frac{1}{r^5} \left( 14 (\hat{n} \cdot \vec{v}_2)^2 (\hat{n} \cdot \vec{S}_1)^2 - 35 \hat{n} \cdot \vec{v}_1 \hat{n} \cdot \vec{v}_2 (\hat{n} \cdot \vec{S}_1)^2 + 5 \vec{v}_1 \cdot \vec{v}_2 (\hat{n} \cdot \vec{S}_1)^2 - \right. \right. \\ & \quad \left. \left. 2 \vec{v}_2 \cdot \vec{v}_2 (\hat{n} \cdot \vec{S}_1)^2 + 10 \hat{n} \cdot \vec{v}_2 \vec{S}_1 \cdot \vec{v}_1 \hat{n} \cdot \vec{S}_1 + 10 \hat{n} \cdot \vec{v}_1 \vec{S}_1 \cdot \vec{v}_2 \hat{n} \cdot \vec{S}_1 - 8 \hat{n} \cdot \vec{v}_2 \vec{S}_1 \cdot \vec{v}_2 \hat{n} \cdot \vec{S}_1 + \frac{4}{5} (\vec{S}_1 \cdot \vec{v}_2)^2 - \right. \right. \\ & \quad \left. \left. 2 (\hat{n} \cdot \vec{v}_2)^2 \vec{S}_1 \cdot \vec{S}_1 + 5 \hat{n} \cdot \vec{v}_1 \hat{n} \cdot \vec{v}_2 \vec{S}_1 \cdot \vec{S}_1 - 2 \vec{S}_1 \cdot \vec{v}_1 \vec{S}_1 \cdot \vec{v}_2 - \vec{S}_1 \cdot \vec{S}_1 \vec{v}_1 \cdot \vec{v}_2 + \frac{2}{5} \vec{S}_1 \cdot \vec{S}_1 \vec{v}_2 \cdot \vec{v}_2 \right) \right) \Bigg\} C_{ES^2 1} \Bigg\} \end{aligned}$$

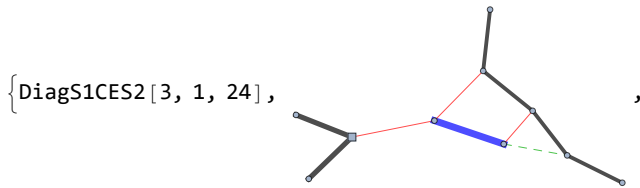

$$\begin{aligned} & \frac{1}{m_1} G^3 m_2^3 C_{ES^2 1} \left( \frac{30 \hat{n} \cdot \vec{a}_2 (\hat{n} \cdot \vec{S}_1)^2 - 12 \vec{S}_1 \cdot \vec{a}_2 \hat{n} \cdot \vec{S}_1 - 6 \vec{S}_1 \cdot \vec{S}_1 \hat{n} \cdot \vec{a}_2}{r^4 \epsilon_d} + \right. \\ & \quad \left. \frac{\log \left( \frac{r}{R_0} \right) (-90 \hat{n} \cdot \vec{a}_2 (\hat{n} \cdot \vec{S}_1)^2 + 36 \vec{S}_1 \cdot \vec{a}_2 \hat{n} \cdot \vec{S}_1 + 18 \vec{S}_1 \cdot \vec{S}_1 \hat{n} \cdot \vec{a}_2)}{r^4} + \right. \end{aligned}$$

$$\left. \frac{123 \hat{n} \cdot \vec{a}_2 \left( \hat{n} \cdot \vec{S}_1 \right)^2 - 42 \vec{S}_1 \cdot \vec{a}_2 \hat{n} \cdot \vec{S}_1 - 39 \vec{S}_1 \cdot \vec{S}_1 \hat{n} \cdot \vec{a}_2}{r^4} \right\}$$

$$\left\{ \text{DiagS1CES2}[3, 1, 25], \right. , G^3 m_1 m_2 C_{\text{ES}^2 1}$$

$$\left( \frac{1}{\epsilon_d} \left( \frac{1}{r^5} \left( \frac{5}{3} \left( \hat{n} \cdot \vec{S}_1 \right)^2 \left( \hat{n} \cdot \vec{v}_1 \right)^2 - \frac{5}{21} \vec{v}_1 \cdot \vec{v}_1 \left( \hat{n} \cdot \vec{S}_1 \right)^2 - \frac{20}{21} \hat{n} \cdot \vec{S}_1 \hat{n} \cdot \vec{v}_1 \vec{S}_1 \cdot \vec{v}_1 - \frac{5}{21} \vec{S}_1 \cdot \vec{S}_1 \left( \hat{n} \cdot \vec{v}_1 \right)^2 + \frac{2}{21} \left( \vec{S}_1 \cdot \vec{v}_1 \right)^2 + \right. \right. \right. \\ \left. \left. \frac{1}{21} \vec{S}_1 \cdot \vec{S}_1 \vec{v}_1 \cdot \vec{v}_1 \right) + \frac{-\frac{6}{7} \hat{n} \cdot \vec{S}_1 \hat{n} \cdot \vec{S}_1 \hat{n} \cdot \vec{v}_1 + \frac{6}{35} \vec{S}_1 \cdot \vec{S}_1 \hat{n} \cdot \vec{v}_1 + \frac{6}{35} \hat{n} \cdot \vec{S}_1 \vec{S}_1 \cdot \vec{v}_1 + \frac{6}{35} \hat{n} \cdot \vec{S}_1 \vec{S}_1 \cdot \vec{v}_1}{r^4} \right) + \right. \\ \left. \frac{1}{r^5} \left( \frac{16}{3} \left( \hat{n} \cdot \vec{S}_1 \right)^2 \left( \hat{n} \cdot \vec{v}_1 \right)^2 + \frac{127}{147} \vec{v}_1 \cdot \vec{v}_1 \left( \hat{n} \cdot \vec{S}_1 \right)^2 - \frac{374}{147} \hat{n} \cdot \vec{S}_1 \hat{n} \cdot \vec{v}_1 \vec{S}_1 \cdot \vec{v}_1 - \frac{160}{147} \vec{S}_1 \cdot \vec{S}_1 \left( \hat{n} \cdot \vec{v}_1 \right)^2 + \right. \right. \\ \left. \left. \frac{22}{147} \left( \vec{S}_1 \cdot \vec{v}_1 \right)^2 - \frac{15}{49} \vec{S}_1 \cdot \vec{S}_1 \vec{v}_1 \cdot \vec{v}_1 \right) + \frac{-\frac{122}{49} \hat{n} \cdot \vec{S}_1 \hat{n} \cdot \vec{S}_1 \hat{n} \cdot \vec{v}_1 + \frac{1464 \vec{S}_1 \cdot \vec{S}_1 \hat{n} \cdot \vec{v}_1}{1225} - \frac{461 \hat{n} \cdot \vec{S}_1 \vec{S}_1 \cdot \vec{v}_1}{1225} - \frac{461 \hat{n} \cdot \vec{S}_1 \vec{S}_1 \cdot \vec{v}_1}{1225}}{r^4} + \right. \\ \left. \log \left( \frac{r}{R_\theta} \right) \left( \frac{1}{r^5} \left( -5 \left( \hat{n} \cdot \vec{S}_1 \right)^2 \left( \hat{n} \cdot \vec{v}_1 \right)^2 + \frac{5}{7} \vec{v}_1 \cdot \vec{v}_1 \left( \hat{n} \cdot \vec{S}_1 \right)^2 + \frac{20}{7} \hat{n} \cdot \vec{S}_1 \hat{n} \cdot \vec{v}_1 \vec{S}_1 \cdot \vec{v}_1 + \frac{5}{7} \vec{S}_1 \cdot \vec{S}_1 \left( \hat{n} \cdot \vec{v}_1 \right)^2 - \frac{2}{7} \right. \right. \right. \\ \left. \left. \left( \vec{S}_1 \cdot \vec{v}_1 \right)^2 - \frac{1}{7} \vec{S}_1 \cdot \vec{S}_1 \vec{v}_1 \cdot \vec{v}_1 \right) + \frac{\frac{18}{7} \hat{n} \cdot \vec{S}_1 \hat{n} \cdot \vec{S}_1 \hat{n} \cdot \vec{v}_1 - \frac{18}{35} \vec{S}_1 \cdot \vec{S}_1 \hat{n} \cdot \vec{v}_1 - \frac{18}{35} \hat{n} \cdot \vec{S}_1 \vec{S}_1 \cdot \vec{v}_1 - \frac{18}{35} \hat{n} \cdot \vec{S}_1 \vec{S}_1 \cdot \vec{v}_1}{r^4} \right) \right) \Bigg\}$$

$$\left\{ \text{DiagS1CES2}[3, 1, 26], \right.$$

$$G^3 m_1 m_2 C_{\text{ES}^2 1} \left( \frac{1}{r^5 \epsilon_d} \left( -3 \left( \hat{n} \cdot \vec{S}_1 \right)^2 \hat{n} \cdot \vec{v}_1 \hat{n} \cdot \vec{v}_2 + \frac{3}{7} \vec{v}_1 \cdot \vec{v}_2 \left( \hat{n} \cdot \vec{S}_1 \right)^2 + \frac{6}{7} \hat{n} \cdot \vec{S}_1 \hat{n} \cdot \vec{v}_2 \vec{S}_1 \cdot \vec{v}_1 + \right. \right. \\ \left. \left. \frac{6}{7} \hat{n} \cdot \vec{S}_1 \hat{n} \cdot \vec{v}_1 \vec{S}_1 \cdot \vec{v}_2 + \frac{3}{7} \vec{S}_1 \cdot \vec{S}_1 \hat{n} \cdot \vec{v}_1 \hat{n} \cdot \vec{v}_2 - \frac{6}{35} \vec{S}_1 \cdot \vec{v}_1 \vec{S}_1 \cdot \vec{v}_2 - \frac{3}{35} \vec{S}_1 \cdot \vec{S}_1 \vec{v}_1 \cdot \vec{v}_2 \right) + \right. \\ \left. \frac{1}{r^5} \log \left( \frac{r}{R_\theta} \right) \left( 9 \left( \hat{n} \cdot \vec{S}_1 \right)^2 \hat{n} \cdot \vec{v}_1 \hat{n} \cdot \vec{v}_2 - \frac{9}{7} \vec{v}_1 \cdot \vec{v}_2 \left( \hat{n} \cdot \vec{S}_1 \right)^2 - \frac{18}{7} \hat{n} \cdot \vec{S}_1 \hat{n} \cdot \vec{v}_2 \vec{S}_1 \cdot \vec{v}_1 - \right. \right. \\ \left. \left. \frac{18}{7} \hat{n} \cdot \vec{S}_1 \hat{n} \cdot \vec{v}_1 \vec{S}_1 \cdot \vec{v}_2 - \frac{9}{7} \vec{S}_1 \cdot \vec{S}_1 \hat{n} \cdot \vec{v}_1 \hat{n} \cdot \vec{v}_2 + \frac{18}{35} \vec{S}_1 \cdot \vec{v}_1 \vec{S}_1 \cdot \vec{v}_2 + \frac{9}{35} \vec{S}_1 \cdot \vec{S}_1 \vec{v}_1 \cdot \vec{v}_2 \right) + \frac{1}{r^5} \right. \\ \left. \left( -10 \left( \hat{n} \cdot \vec{S}_1 \right)^2 \hat{n} \cdot \vec{v}_1 \hat{n} \cdot \vec{v}_2 - \frac{23}{49} \vec{v}_1 \cdot \vec{v}_2 \left( \hat{n} \cdot \vec{S}_1 \right)^2 + \frac{38}{49} \hat{n} \cdot \vec{S}_1 \hat{n} \cdot \vec{v}_2 \vec{S}_1 \cdot \vec{v}_1 + \frac{164}{49} \hat{n} \cdot \vec{S}_1 \hat{n} \cdot \vec{v}_1 \vec{S}_1 \cdot \vec{v}_2 + \right. \right. \\ \left. \left. \frac{110}{49} \vec{S}_1 \cdot \vec{S}_1 \hat{n} \cdot \vec{v}_1 \hat{n} \cdot \vec{v}_2 - \frac{274 \vec{S}_1 \cdot \vec{v}_1 \vec{S}_1 \cdot \vec{v}_2}{1225} + \frac{213 \vec{S}_1 \cdot \vec{S}_1 \vec{v}_1 \cdot \vec{v}_2}{1225} \right) \right) \Bigg\}$$

{DiagS1CES2[3, 1, 27],

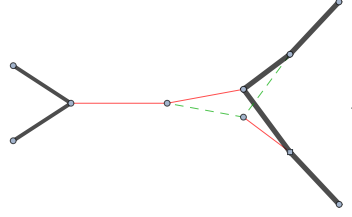

,

$$\begin{aligned}
 G^3 m_1 m_2 \left( \frac{1}{r^5 \in_d} \left( 2 (\hat{n} \cdot \vec{v}_1)^2 (\hat{n} \cdot \vec{S}_1)^2 + 2 \hat{n} \cdot \vec{v}_1 \hat{n} \cdot \vec{v}_2 (\hat{n} \cdot \vec{S}_1)^2 - \frac{2}{7} \vec{v}_1 \cdot \vec{v}_1 (\hat{n} \cdot \vec{S}_1)^2 - \frac{2}{7} \vec{v}_1 \cdot \vec{v}_2 (\hat{n} \cdot \vec{S}_1)^2 - \right. \right. \\
 \frac{8}{7} \hat{n} \cdot \vec{v}_1 \vec{S}_1 \cdot \vec{v}_1 \hat{n} \cdot \vec{S}_1 - \frac{4}{7} \hat{n} \cdot \vec{v}_2 \vec{S}_1 \cdot \vec{v}_1 \hat{n} \cdot \vec{S}_1 - \frac{4}{7} \hat{n} \cdot \vec{v}_1 \vec{S}_1 \cdot \vec{v}_2 \hat{n} \cdot \vec{S}_1 + \frac{4}{35} (\vec{S}_1 \cdot \vec{v}_1)^2 - \\
 \left. \frac{2}{7} (\hat{n} \cdot \vec{v}_1)^2 \vec{S}_1 \cdot \vec{S}_1 - \frac{2}{7} \hat{n} \cdot \vec{v}_1 \hat{n} \cdot \vec{v}_2 \vec{S}_1 \cdot \vec{S}_1 + \frac{4}{35} \vec{S}_1 \cdot \vec{v}_1 \vec{S}_1 \cdot \vec{v}_2 + \frac{2}{35} \vec{S}_1 \cdot \vec{S}_1 \vec{v}_1 \cdot \vec{v}_1 + \frac{2}{35} \vec{S}_1 \cdot \vec{S}_1 \vec{v}_1 \cdot \vec{v}_2 \right) + \\
 \frac{1}{r^5} \left( 7 (\hat{n} \cdot \vec{v}_1)^2 (\hat{n} \cdot \vec{S}_1)^2 + 7 \hat{n} \cdot \vec{v}_1 \hat{n} \cdot \vec{v}_2 (\hat{n} \cdot \vec{S}_1)^2 - \frac{71}{49} \vec{v}_1 \cdot \vec{v}_1 (\hat{n} \cdot \vec{S}_1)^2 - \frac{43}{49} \vec{v}_1 \cdot \vec{v}_2 (\hat{n} \cdot \vec{S}_1)^2 - \right. \\
 \frac{32}{49} \hat{n} \cdot \vec{v}_1 \vec{S}_1 \cdot \vec{v}_1 \hat{n} \cdot \vec{S}_1 + \frac{138}{49} \hat{n} \cdot \vec{v}_2 \vec{S}_1 \cdot \vec{v}_1 \hat{n} \cdot \vec{S}_1 - \frac{86}{49} \hat{n} \cdot \vec{v}_1 \vec{S}_1 \cdot \vec{v}_2 \hat{n} \cdot \vec{S}_1 - \frac{74 (\vec{S}_1 \cdot \vec{v}_1)^2}{1225} - \\
 \left. \frac{113}{49} (\hat{n} \cdot \vec{v}_1)^2 \vec{S}_1 \cdot \vec{S}_1 - \frac{141}{49} \hat{n} \cdot \vec{v}_1 \hat{n} \cdot \vec{v}_2 \vec{S}_1 \cdot \vec{S}_1 - \frac{774 \vec{S}_1 \cdot \vec{v}_1 \vec{S}_1 \cdot \vec{v}_2}{1225} + \frac{663 \vec{S}_1 \cdot \vec{S}_1 \vec{v}_1 \cdot \vec{v}_1}{1225} + \frac{663 \vec{S}_1 \cdot \vec{S}_1 \vec{v}_1 \cdot \vec{v}_2}{1225} \right) + \\
 \frac{1}{r^5} \left( -6 (\hat{n} \cdot \vec{v}_1)^2 (\hat{n} \cdot \vec{S}_1)^2 - 6 \hat{n} \cdot \vec{v}_1 \hat{n} \cdot \vec{v}_2 (\hat{n} \cdot \vec{S}_1)^2 + \frac{6}{7} \vec{v}_1 \cdot \vec{v}_1 (\hat{n} \cdot \vec{S}_1)^2 + \frac{6}{7} \vec{v}_1 \cdot \vec{v}_2 (\hat{n} \cdot \vec{S}_1)^2 + \right. \\
 \frac{24}{7} \hat{n} \cdot \vec{v}_1 \vec{S}_1 \cdot \vec{v}_1 \hat{n} \cdot \vec{S}_1 + \frac{12}{7} \hat{n} \cdot \vec{v}_2 \vec{S}_1 \cdot \vec{v}_1 \hat{n} \cdot \vec{S}_1 + \frac{12}{7} \hat{n} \cdot \vec{v}_1 \vec{S}_1 \cdot \vec{v}_2 \hat{n} \cdot \vec{S}_1 - \frac{12}{35} (\vec{S}_1 \cdot \vec{v}_1)^2 + \frac{6}{7} (\hat{n} \cdot \vec{v}_1)^2 \vec{S}_1 \cdot \vec{S}_1 + \\
 \left. \frac{6}{7} \hat{n} \cdot \vec{v}_1 \hat{n} \cdot \vec{v}_2 \vec{S}_1 \cdot \vec{S}_1 - \frac{12}{35} \vec{S}_1 \cdot \vec{v}_1 \vec{S}_1 \cdot \vec{v}_2 - \frac{6}{35} \vec{S}_1 \cdot \vec{S}_1 \vec{v}_1 \cdot \vec{v}_1 - \frac{6}{35} \vec{S}_1 \cdot \vec{S}_1 \vec{v}_1 \cdot \vec{v}_2 \right) \log \left( \frac{r}{R_\theta} \right) \Bigg\} C_{\text{ES}^2 1}
 \end{aligned}$$

{DiagS1CES2[3, 1, 28],

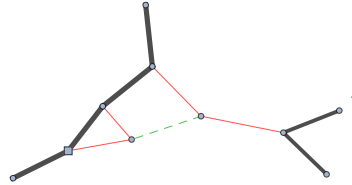

,

$$\begin{aligned}
 G^3 m_1 m_2 \left( \frac{1}{r^4} \left( \frac{123}{98} \hat{n} \cdot \vec{S}_1 \hat{n} \cdot \vec{S}_1 \hat{n} \cdot \vec{v}_1 - \frac{937 \vec{S}_1 \cdot \vec{S}_1 \hat{n} \cdot \vec{v}_1}{2450} - \frac{3}{2} \hat{n} \cdot \vec{S}_1 \hat{n} \cdot \vec{S}_1 \hat{n} \cdot \vec{v}_2 - \right. \right. \\
 \frac{206 \hat{n} \cdot \vec{S}_1 \vec{S}_1 \cdot \vec{v}_1}{1225} + \frac{3}{10} \hat{n} \cdot \vec{S}_1 \vec{S}_1 \cdot \vec{v}_2 + \frac{3}{10} \hat{n} \cdot \vec{v}_2 \vec{S}_1 \cdot \vec{S}_1 - \frac{206 \hat{n} \cdot \vec{S}_1 \vec{S}_1 \cdot \vec{v}_1}{1225} + \frac{3}{10} \hat{n} \cdot \vec{S}_1 \vec{S}_1 \cdot \vec{v}_2 \Bigg) + \frac{1}{r^5} \\
 \left( -\frac{131}{48} (\hat{n} \cdot \vec{v}_1)^2 (\hat{n} \cdot \vec{S}_1)^2 + 8 \hat{n} \cdot \vec{v}_1 \hat{n} \cdot \vec{v}_2 (\hat{n} \cdot \vec{S}_1)^2 + \frac{817 \vec{v}_1 \cdot \vec{v}_1 (\hat{n} \cdot \vec{S}_1)^2}{2352} - \frac{53}{49} \vec{v}_1 \cdot \vec{v}_2 (\hat{n} \cdot \vec{S}_1)^2 + \right. \\
 \left. \frac{649}{588} \hat{n} \cdot \vec{v}_1 \vec{S}_1 \cdot \vec{v}_1 \hat{n} \cdot \vec{S}_1 - \frac{141}{49} \hat{n} \cdot \vec{v}_2 \vec{S}_1 \cdot \vec{v}_1 \hat{n} \cdot \vec{S}_1 - \frac{106}{49} \hat{n} \cdot \vec{v}_1 \vec{S}_1 \cdot \vec{v}_2 \hat{n} \cdot \vec{S}_1 - \frac{2713 (\vec{S}_1 \cdot \vec{v}_1)^2}{29400} + \right.
 \end{aligned}$$

$$\begin{aligned}
& \left. \frac{1517}{2352} (\hat{n} \cdot \vec{v}_1)^2 \vec{S}_1 \cdot \vec{S}_1 - \frac{53}{49} \hat{n} \cdot \vec{v}_1 \hat{n} \cdot \vec{v}_2 \vec{S}_1 \cdot \vec{S}_1 + \frac{663}{1225} \vec{S}_1 \cdot \vec{v}_1 \vec{S}_1 \cdot \vec{v}_2 - \frac{2071}{19600} \vec{S}_1 \cdot \vec{S}_1 \vec{v}_1 \cdot \vec{v}_1 + \frac{244}{1225} \vec{S}_1 \cdot \vec{S}_1 \vec{v}_1 \cdot \vec{v}_2 \right) + \\
& \left( \frac{-\frac{12}{7} \hat{n} \cdot \vec{S}_1 \hat{n} \cdot \vec{S}_1 \hat{n} \cdot \vec{v}_1 + \frac{12}{35} \vec{S}_1 \cdot \vec{S}_1 \hat{n} \cdot \vec{v}_1 + \frac{12}{35} \hat{n} \cdot \vec{S}_1 \vec{S}_1 \cdot \vec{v}_1 + \frac{12}{35} \hat{n} \cdot \vec{S}_1 \vec{S}_1 \cdot \vec{v}_1}{r^4} + \frac{1}{r^5} \right. \\
& \left( \frac{13}{4} (\hat{n} \cdot \vec{v}_1)^2 (\hat{n} \cdot \vec{S}_1)^2 - 3 \hat{n} \cdot \vec{v}_1 \hat{n} \cdot \vec{v}_2 (\hat{n} \cdot \vec{S}_1)^2 - \frac{13}{28} \vec{v}_1 \cdot \vec{v}_1 (\hat{n} \cdot \vec{S}_1)^2 + \frac{3}{7} \vec{v}_1 \cdot \vec{v}_2 (\hat{n} \cdot \vec{S}_1)^2 - \right. \\
& \left. \frac{13}{7} \hat{n} \cdot \vec{v}_1 \vec{S}_1 \cdot \vec{v}_1 \hat{n} \cdot \vec{S}_1 + \frac{6}{7} \hat{n} \cdot \vec{v}_2 \vec{S}_1 \cdot \vec{v}_1 \hat{n} \cdot \vec{S}_1 + \frac{6}{7} \hat{n} \cdot \vec{v}_1 \vec{S}_1 \cdot \vec{v}_2 \hat{n} \cdot \vec{S}_1 + \frac{13}{70} (\vec{S}_1 \cdot \vec{v}_1)^2 - \frac{13}{28} (\hat{n} \cdot \vec{v}_1)^2 \vec{S}_1 \cdot \vec{S}_1 + \right. \\
& \left. \frac{3}{7} \hat{n} \cdot \vec{v}_1 \hat{n} \cdot \vec{v}_2 \vec{S}_1 \cdot \vec{S}_1 - \frac{6}{35} \vec{S}_1 \cdot \vec{v}_1 \vec{S}_1 \cdot \vec{v}_2 + \frac{13}{140} \vec{S}_1 \cdot \vec{S}_1 \vec{v}_1 \cdot \vec{v}_1 - \frac{3}{35} \vec{S}_1 \cdot \vec{S}_1 \vec{v}_1 \cdot \vec{v}_2 \right) \log \left( \frac{r}{R_\theta} \right) + \\
& \frac{1}{\epsilon_d} \left( \frac{\frac{4}{7} \hat{n} \cdot \vec{S}_1 \hat{n} \cdot \vec{S}_1 \hat{n} \cdot \vec{v}_1 - \frac{4}{35} \vec{S}_1 \cdot \vec{S}_1 \hat{n} \cdot \vec{v}_1 - \frac{4}{35} \hat{n} \cdot \vec{S}_1 \vec{S}_1 \cdot \vec{v}_1 - \frac{4}{35} \hat{n} \cdot \vec{S}_1 \vec{S}_1 \cdot \vec{v}_1}{r^4} + \frac{1}{r^5} \right. \\
& \left( -\frac{13}{12} (\hat{n} \cdot \vec{v}_1)^2 (\hat{n} \cdot \vec{S}_1)^2 + \hat{n} \cdot \vec{v}_1 \hat{n} \cdot \vec{v}_2 (\hat{n} \cdot \vec{S}_1)^2 + \frac{13}{84} \vec{v}_1 \cdot \vec{v}_1 (\hat{n} \cdot \vec{S}_1)^2 - \frac{1}{7} \vec{v}_1 \cdot \vec{v}_2 (\hat{n} \cdot \vec{S}_1)^2 + \right. \\
& \left. \frac{13}{21} \hat{n} \cdot \vec{v}_1 \vec{S}_1 \cdot \vec{v}_1 \hat{n} \cdot \vec{S}_1 - \frac{2}{7} \hat{n} \cdot \vec{v}_2 \vec{S}_1 \cdot \vec{v}_1 \hat{n} \cdot \vec{S}_1 - \frac{2}{7} \hat{n} \cdot \vec{v}_1 \vec{S}_1 \cdot \vec{v}_2 \hat{n} \cdot \vec{S}_1 - \frac{13}{210} (\vec{S}_1 \cdot \vec{v}_1)^2 + \frac{13}{84} (\hat{n} \cdot \vec{v}_1)^2 \vec{S}_1 \cdot \vec{S}_1 - \right. \\
& \left. \left. \frac{1}{7} \hat{n} \cdot \vec{v}_1 \hat{n} \cdot \vec{v}_2 \vec{S}_1 \cdot \vec{S}_1 + \frac{2}{35} \vec{S}_1 \cdot \vec{v}_1 \vec{S}_1 \cdot \vec{v}_2 - \frac{13}{420} \vec{S}_1 \cdot \vec{S}_1 \vec{v}_1 \cdot \vec{v}_1 + \frac{1}{35} \vec{S}_1 \cdot \vec{S}_1 \vec{v}_1 \cdot \vec{v}_2 \right) \right) \Bigg\} C_{ES^2_1} \}
\end{aligned}$$

$\{\text{DiagS1CES2}[3, 1, 29],$ 
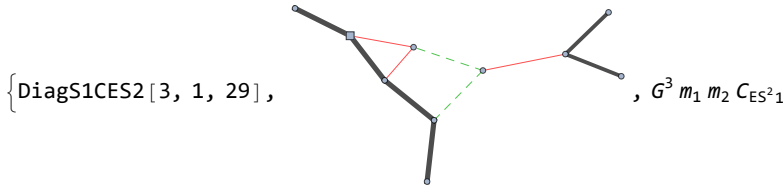
 $, G^3 m_1 m_2 C_{ES^2_1}$

$$\begin{aligned}
& \left( \frac{1}{\epsilon_d} \left( \frac{1}{r^5} \left( \frac{5}{3} (\hat{n} \cdot \vec{S}_1)^2 (\hat{n} \cdot \vec{v}_1)^2 - \frac{5}{21} \vec{v}_1 \cdot \vec{v}_1 (\hat{n} \cdot \vec{S}_1)^2 - \frac{20}{21} \hat{n} \cdot \vec{S}_1 \hat{n} \cdot \vec{v}_1 \vec{S}_1 \cdot \vec{v}_1 - \frac{5}{21} \vec{S}_1 \cdot \vec{S}_1 (\hat{n} \cdot \vec{v}_1)^2 + \frac{2}{21} (\vec{S}_1 \cdot \vec{v}_1)^2 + \right. \right. \right. \\
& \left. \left. \frac{1}{21} \vec{S}_1 \cdot \vec{S}_1 \vec{v}_1 \cdot \vec{v}_1 \right) + \frac{-\frac{4}{7} \hat{n} \cdot \vec{S}_1 \hat{n} \cdot \vec{S}_1 \hat{n} \cdot \vec{v}_1 + \frac{4}{35} \vec{S}_1 \cdot \vec{S}_1 \hat{n} \cdot \vec{v}_1 + \frac{4}{35} \hat{n} \cdot \vec{S}_1 \vec{S}_1 \cdot \vec{v}_1 + \frac{4}{35} \hat{n} \cdot \vec{S}_1 \vec{S}_1 \cdot \vec{v}_1}{r^4} \right) + \\
& \frac{1}{r^5} \left( \frac{23}{4} (\hat{n} \cdot \vec{S}_1)^2 (\hat{n} \cdot \vec{v}_1)^2 + \frac{641}{588} \vec{v}_1 \cdot \vec{v}_1 (\hat{n} \cdot \vec{S}_1)^2 - \frac{283}{147} \hat{n} \cdot \vec{S}_1 \hat{n} \cdot \vec{v}_1 \vec{S}_1 \cdot \vec{v}_1 - \frac{281}{196} \vec{S}_1 \cdot \vec{S}_1 (\hat{n} \cdot \vec{v}_1)^2 - \right. \\
& \left. \frac{11}{98} (\vec{S}_1 \cdot \vec{v}_1)^2 - \frac{173}{588} \vec{S}_1 \cdot \vec{S}_1 \vec{v}_1 \cdot \vec{v}_1 \right) + \frac{-\frac{86}{49} \hat{n} \cdot \vec{S}_1 \hat{n} \cdot \vec{S}_1 \hat{n} \cdot \vec{v}_1 + \frac{1326}{1225} \vec{S}_1 \cdot \vec{S}_1 \hat{n} \cdot \vec{v}_1 - \frac{774}{1225} \hat{n} \cdot \vec{S}_1 \vec{S}_1 \cdot \vec{v}_1 - \frac{774}{1225} \hat{n} \cdot \vec{S}_1 \vec{S}_1 \cdot \vec{v}_1}{r^4} + \\
& \log \left( \frac{r}{R_\theta} \right) \left( \frac{1}{r^5} \left( -5 (\hat{n} \cdot \vec{S}_1)^2 (\hat{n} \cdot \vec{v}_1)^2 + \frac{5}{7} \vec{v}_1 \cdot \vec{v}_1 (\hat{n} \cdot \vec{S}_1)^2 + \frac{20}{7} \hat{n} \cdot \vec{S}_1 \hat{n} \cdot \vec{v}_1 \vec{S}_1 \cdot \vec{v}_1 + \frac{5}{7} \vec{S}_1 \cdot \vec{S}_1 (\hat{n} \cdot \vec{v}_1)^2 - \frac{2}{7} \right. \right.
\end{aligned}$$

$$\left. \left( \vec{S}_1 \cdot \vec{v}_1 \right)^2 - \frac{1}{7} \vec{S}_1 \cdot \vec{S}_1 \vec{v}_1 \cdot \vec{v}_1 \right) + \frac{\frac{12}{7} \hat{n} \cdot \vec{S}_1 \hat{n} \cdot \vec{S}_1 \hat{n} \cdot \vec{v}_1 - \frac{12}{35} \vec{S}_1 \cdot \vec{S}_1 \hat{n} \cdot \vec{v}_1 - \frac{12}{35} \hat{n} \cdot \vec{S}_1 \vec{S}_1 \cdot \vec{v}_1 - \frac{12}{35} \hat{n} \cdot \vec{S}_1 \vec{S}_1 \cdot \vec{v}_1}{r^4} \right\}$$

{DiagS1CES2[3, 1, 30],

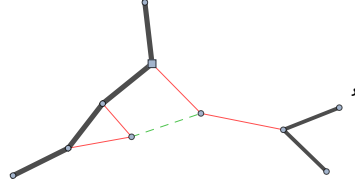

$$G^3 m_1 m_2 \left( \frac{\frac{97}{98} \hat{n} \cdot \vec{S}_1 \hat{n} \cdot \vec{S}_1 \hat{n} \cdot \vec{v}_1 - \frac{723 \vec{S}_1 \cdot \vec{S}_1 \hat{n} \cdot \vec{v}_1}{2450} - \frac{274 \hat{n} \cdot \vec{S}_1 \vec{S}_1 \cdot \vec{v}_1}{1225} - \frac{274 \hat{n} \cdot \vec{S}_1 \vec{S}_1 \cdot \vec{v}_1}{1225}}{r^4} + \frac{1}{r^5} \right.$$

$$\left( -\frac{65}{24} (\hat{n} \cdot \vec{v}_1)^2 (\hat{n} \cdot \vec{S}_1)^2 + \frac{1}{4} \hat{n} \cdot \vec{v}_1 \hat{n} \cdot \vec{v}_2 (\hat{n} \cdot \vec{S}_1)^2 + \frac{195}{392} \vec{v}_1 \cdot \vec{v}_1 (\hat{n} \cdot \vec{S}_1)^2 - \frac{25}{196} \vec{v}_1 \cdot \vec{v}_2 (\hat{n} \cdot \vec{S}_1)^2 + \right.$$

$$\frac{153}{98} \hat{n} \cdot \vec{v}_1 \vec{S}_1 \cdot \vec{v}_1 \hat{n} \cdot \vec{S}_1 + \frac{40}{49} \hat{n} \cdot \vec{v}_2 \vec{S}_1 \cdot \vec{v}_1 \hat{n} \cdot \vec{S}_1 - \frac{25}{98} \hat{n} \cdot \vec{v}_1 \vec{S}_1 \cdot \vec{v}_2 \hat{n} \cdot \vec{S}_1 - \frac{103}{588} (\vec{S}_1 \cdot \vec{v}_1)^2 +$$

$$\left. \frac{683 (\hat{n} \cdot \vec{v}_1)^2 \vec{S}_1 \cdot \vec{S}_1}{1176} - \frac{25}{196} \hat{n} \cdot \vec{v}_1 \hat{n} \cdot \vec{v}_2 \vec{S}_1 \cdot \vec{S}_1 - \frac{137 \vec{S}_1 \cdot \vec{v}_1 \vec{S}_1 \cdot \vec{v}_2}{1225} - \frac{173 \vec{S}_1 \cdot \vec{S}_1 \vec{v}_1 \cdot \vec{v}_1}{1176} + \frac{251 \vec{S}_1 \cdot \vec{S}_1 \vec{v}_1 \cdot \vec{v}_2}{4900} \right) +$$

$$\left( \frac{-\frac{18}{7} \hat{n} \cdot \vec{S}_1 \hat{n} \cdot \vec{S}_1 \hat{n} \cdot \vec{v}_1 + \frac{18}{35} \vec{S}_1 \cdot \vec{S}_1 \hat{n} \cdot \vec{v}_1 + \frac{18}{35} \hat{n} \cdot \vec{S}_1 \vec{S}_1 \cdot \vec{v}_1 + \frac{18}{35} \hat{n} \cdot \vec{S}_1 \vec{S}_1 \cdot \vec{v}_1}{r^4} + \frac{1}{r^5} \right.$$

$$\left( \frac{25}{4} (\hat{n} \cdot \vec{v}_1)^2 (\hat{n} \cdot \vec{S}_1)^2 + \frac{9}{2} \hat{n} \cdot \vec{v}_1 \hat{n} \cdot \vec{v}_2 (\hat{n} \cdot \vec{S}_1)^2 - \frac{25}{28} \vec{v}_1 \cdot \vec{v}_1 (\hat{n} \cdot \vec{S}_1)^2 - \frac{9}{14} \vec{v}_1 \cdot \vec{v}_2 (\hat{n} \cdot \vec{S}_1)^2 - \right.$$

$$\frac{25}{7} \hat{n} \cdot \vec{v}_1 \vec{S}_1 \cdot \vec{v}_1 \hat{n} \cdot \vec{S}_1 - \frac{9}{7} \hat{n} \cdot \vec{v}_2 \vec{S}_1 \cdot \vec{v}_1 \hat{n} \cdot \vec{S}_1 - \frac{9}{7} \hat{n} \cdot \vec{v}_1 \vec{S}_1 \cdot \vec{v}_2 \hat{n} \cdot \vec{S}_1 + \frac{5}{14} (\vec{S}_1 \cdot \vec{v}_1)^2 - \frac{25}{28} (\hat{n} \cdot \vec{v}_1)^2 \vec{S}_1 \cdot \vec{S}_1 -$$

$$\left. \frac{9}{14} \hat{n} \cdot \vec{v}_1 \hat{n} \cdot \vec{v}_2 \vec{S}_1 \cdot \vec{S}_1 + \frac{9}{35} \vec{S}_1 \cdot \vec{v}_1 \vec{S}_1 \cdot \vec{v}_2 + \frac{5}{28} \vec{S}_1 \cdot \vec{S}_1 \vec{v}_1 \cdot \vec{v}_1 + \frac{9}{70} \vec{S}_1 \cdot \vec{S}_1 \vec{v}_1 \cdot \vec{v}_2 \right) \log \left( \frac{r}{R_\theta} \right) +$$

$$\frac{1}{\epsilon_d} \left( \frac{\frac{6}{7} \hat{n} \cdot \vec{S}_1 \hat{n} \cdot \vec{S}_1 \hat{n} \cdot \vec{v}_1 - \frac{6}{35} \vec{S}_1 \cdot \vec{S}_1 \hat{n} \cdot \vec{v}_1 - \frac{6}{35} \hat{n} \cdot \vec{S}_1 \vec{S}_1 \cdot \vec{v}_1 - \frac{6}{35} \hat{n} \cdot \vec{S}_1 \vec{S}_1 \cdot \vec{v}_1}{r^4} + \frac{1}{r^5} \right.$$

$$\left( -\frac{25}{12} (\hat{n} \cdot \vec{v}_1)^2 (\hat{n} \cdot \vec{S}_1)^2 - \frac{3}{2} \hat{n} \cdot \vec{v}_1 \hat{n} \cdot \vec{v}_2 (\hat{n} \cdot \vec{S}_1)^2 + \frac{25}{84} \vec{v}_1 \cdot \vec{v}_1 (\hat{n} \cdot \vec{S}_1)^2 + \frac{3}{14} \vec{v}_1 \cdot \vec{v}_2 (\hat{n} \cdot \vec{S}_1)^2 + \right.$$

$$\frac{25}{21} \hat{n} \cdot \vec{v}_1 \vec{S}_1 \cdot \vec{v}_1 \hat{n} \cdot \vec{S}_1 + \frac{3}{7} \hat{n} \cdot \vec{v}_2 \vec{S}_1 \cdot \vec{v}_1 \hat{n} \cdot \vec{S}_1 + \frac{3}{7} \hat{n} \cdot \vec{v}_1 \vec{S}_1 \cdot \vec{v}_2 \hat{n} \cdot \vec{S}_1 - \frac{5}{42} (\vec{S}_1 \cdot \vec{v}_1)^2 + \frac{25}{84} (\hat{n} \cdot \vec{v}_1)^2 \vec{S}_1 \cdot \vec{S}_1 +$$

$$\left. \frac{3}{14} \hat{n} \cdot \vec{v}_1 \hat{n} \cdot \vec{v}_2 \vec{S}_1 \cdot \vec{S}_1 - \frac{3}{35} \vec{S}_1 \cdot \vec{v}_1 \vec{S}_1 \cdot \vec{v}_2 - \frac{5}{84} \vec{S}_1 \cdot \vec{S}_1 \vec{v}_1 \cdot \vec{v}_1 - \frac{3}{70} \vec{S}_1 \cdot \vec{S}_1 \vec{v}_1 \cdot \vec{v}_2 \right) \Bigg\} c_{ES^2 1}$$

{DiagS1CES2[3, 1, 31],

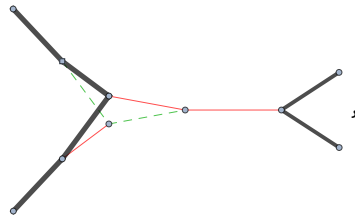

$$\begin{aligned}
& G^3 m_1 m_2 \left( \frac{1}{r^4} \left( -14 \hat{n} \cdot \vec{S}_1 \hat{n} \cdot \vec{S}_1 \hat{n} \cdot \vec{v}_1 + \frac{112}{25} \vec{S}_1 \cdot \vec{S}_1 \hat{n} \cdot \vec{v}_1 - 14 \hat{n} \cdot \vec{S}_1 \hat{n} \cdot \vec{S}_1 \hat{n} \cdot \vec{v}_2 + \right. \right. \\
& \quad \left. \frac{37}{25} \hat{n} \cdot \vec{S}_1 \vec{S}_1 \cdot \vec{v}_1 + \frac{52}{25} \hat{n} \cdot \vec{S}_1 \vec{S}_1 \cdot \vec{v}_2 + \frac{102}{25} \hat{n} \cdot \vec{v}_2 \vec{S}_1 \cdot \vec{S}_1 + \frac{37}{25} \hat{n} \cdot \vec{S}_1 \vec{S}_1 \cdot \vec{v}_1 + \frac{52}{25} \hat{n} \cdot \vec{S}_1 \vec{S}_1 \cdot \vec{v}_2 \right) + \frac{1}{r^5} \\
& \quad \left( 27 (\hat{n} \cdot \vec{v}_1)^2 (\hat{n} \cdot \vec{S}_1)^2 + 27 \hat{n} \cdot \vec{v}_1 \hat{n} \cdot \vec{v}_2 (\hat{n} \cdot \vec{S}_1)^2 - \frac{131}{49} \vec{v}_1 \cdot \vec{v}_1 (\hat{n} \cdot \vec{S}_1)^2 - \frac{159}{49} \vec{v}_1 \cdot \vec{v}_2 (\hat{n} \cdot \vec{S}_1)^2 - \right. \\
& \quad \frac{608}{49} \hat{n} \cdot \vec{v}_1 \vec{S}_1 \cdot \vec{v}_1 \hat{n} \cdot \vec{S}_1 - \frac{374}{49} \hat{n} \cdot \vec{v}_2 \vec{S}_1 \cdot \vec{v}_1 \hat{n} \cdot \vec{S}_1 - \frac{318}{49} \hat{n} \cdot \vec{v}_1 \vec{S}_1 \cdot \vec{v}_2 \hat{n} \cdot \vec{S}_1 + \frac{30}{49} (\vec{S}_1 \cdot \vec{v}_1)^2 - \\
& \quad \frac{285}{49} (\hat{n} \cdot \vec{v}_1)^2 \vec{S}_1 \cdot \vec{S}_1 - \frac{257}{49} \hat{n} \cdot \vec{v}_1 \hat{n} \cdot \vec{v}_2 \vec{S}_1 \cdot \vec{S}_1 + \frac{58}{49} \vec{S}_1 \cdot \vec{v}_1 \vec{S}_1 \cdot \vec{v}_2 + \frac{43}{49} \vec{S}_1 \cdot \vec{S}_1 \vec{v}_1 \cdot \vec{v}_1 + \frac{43}{49} \vec{S}_1 \cdot \vec{S}_1 \vec{v}_1 \cdot \vec{v}_2 \Big) + \\
& \quad \left( \frac{1}{r^4} \left( 18 \hat{n} \cdot \vec{S}_1 \hat{n} \cdot \vec{S}_1 \hat{n} \cdot \vec{v}_1 - \frac{18}{5} \vec{S}_1 \cdot \vec{S}_1 \hat{n} \cdot \vec{v}_1 + 18 \hat{n} \cdot \vec{S}_1 \hat{n} \cdot \vec{S}_1 \hat{n} \cdot \vec{v}_2 - \frac{18}{5} \hat{n} \cdot \vec{S}_1 \vec{S}_1 \cdot \vec{v}_1 - \right. \right. \\
& \quad \left. \frac{18}{5} \hat{n} \cdot \vec{S}_1 \vec{S}_1 \cdot \vec{v}_2 - \frac{18}{5} \hat{n} \cdot \vec{v}_2 \vec{S}_1 \cdot \vec{S}_1 - \frac{18}{5} \hat{n} \cdot \vec{S}_1 \vec{S}_1 \cdot \vec{v}_1 - \frac{18}{5} \hat{n} \cdot \vec{S}_1 \vec{S}_1 \cdot \vec{v}_2 \right) + \frac{1}{r^5} \\
& \quad \left( -30 (\hat{n} \cdot \vec{v}_1)^2 (\hat{n} \cdot \vec{S}_1)^2 - 30 \hat{n} \cdot \vec{v}_1 \hat{n} \cdot \vec{v}_2 (\hat{n} \cdot \vec{S}_1)^2 + \frac{30}{7} \vec{v}_1 \cdot \vec{v}_1 (\hat{n} \cdot \vec{S}_1)^2 + \frac{30}{7} \vec{v}_1 \cdot \vec{v}_2 (\hat{n} \cdot \vec{S}_1)^2 + \right. \\
& \quad \frac{120}{7} \hat{n} \cdot \vec{v}_1 \vec{S}_1 \cdot \vec{v}_1 \hat{n} \cdot \vec{S}_1 + \frac{60}{7} \hat{n} \cdot \vec{v}_2 \vec{S}_1 \cdot \vec{v}_1 \hat{n} \cdot \vec{S}_1 + \frac{60}{7} \hat{n} \cdot \vec{v}_1 \vec{S}_1 \cdot \vec{v}_2 \hat{n} \cdot \vec{S}_1 - \frac{12}{7} (\vec{S}_1 \cdot \vec{v}_1)^2 + \\
& \quad \left. \frac{30}{7} (\hat{n} \cdot \vec{v}_1)^2 \vec{S}_1 \cdot \vec{S}_1 + \frac{30}{7} \hat{n} \cdot \vec{v}_1 \hat{n} \cdot \vec{v}_2 \vec{S}_1 \cdot \vec{S}_1 - \frac{12}{7} \vec{S}_1 \cdot \vec{v}_1 \vec{S}_1 \cdot \vec{v}_2 - \frac{6}{7} \vec{S}_1 \cdot \vec{S}_1 \vec{v}_1 \cdot \vec{v}_1 - \frac{6}{7} \vec{S}_1 \cdot \vec{S}_1 \vec{v}_1 \cdot \vec{v}_2 \right) \Big) \Big) \Big) C_{ES^2_1} \Big\} \\
& \log \left( \frac{r}{R_0} \right) + \frac{1}{\epsilon_d} \left( \frac{1}{r^4} \left( -6 \hat{n} \cdot \vec{S}_1 \hat{n} \cdot \vec{S}_1 \hat{n} \cdot \vec{v}_1 + \frac{6}{5} \vec{S}_1 \cdot \vec{S}_1 \hat{n} \cdot \vec{v}_1 - 6 \hat{n} \cdot \vec{S}_1 \hat{n} \cdot \vec{S}_1 \hat{n} \cdot \vec{v}_2 + \frac{6}{5} \hat{n} \cdot \vec{S}_1 \vec{S}_1 \cdot \vec{v}_1 + \right. \right. \\
& \quad \left. \frac{6}{5} \hat{n} \cdot \vec{S}_1 \vec{S}_1 \cdot \vec{v}_2 + \frac{6}{5} \hat{n} \cdot \vec{v}_2 \vec{S}_1 \cdot \vec{S}_1 + \frac{6}{5} \hat{n} \cdot \vec{S}_1 \vec{S}_1 \cdot \vec{v}_1 + \frac{6}{5} \hat{n} \cdot \vec{S}_1 \vec{S}_1 \cdot \vec{v}_2 \right) + \frac{1}{r^5} \\
& \quad \left( 10 (\hat{n} \cdot \vec{v}_1)^2 (\hat{n} \cdot \vec{S}_1)^2 + 10 \hat{n} \cdot \vec{v}_1 \hat{n} \cdot \vec{v}_2 (\hat{n} \cdot \vec{S}_1)^2 - \frac{10}{7} \vec{v}_1 \cdot \vec{v}_1 (\hat{n} \cdot \vec{S}_1)^2 - \frac{10}{7} \vec{v}_1 \cdot \vec{v}_2 (\hat{n} \cdot \vec{S}_1)^2 - \right. \\
& \quad \frac{40}{7} \hat{n} \cdot \vec{v}_1 \vec{S}_1 \cdot \vec{v}_1 \hat{n} \cdot \vec{S}_1 - \frac{20}{7} \hat{n} \cdot \vec{v}_2 \vec{S}_1 \cdot \vec{v}_1 \hat{n} \cdot \vec{S}_1 - \frac{20}{7} \hat{n} \cdot \vec{v}_1 \vec{S}_1 \cdot \vec{v}_2 \hat{n} \cdot \vec{S}_1 + \frac{4}{7} (\vec{S}_1 \cdot \vec{v}_1)^2 - \\
& \quad \left. \frac{10}{7} (\hat{n} \cdot \vec{v}_1)^2 \vec{S}_1 \cdot \vec{S}_1 - \frac{10}{7} \hat{n} \cdot \vec{v}_1 \hat{n} \cdot \vec{v}_2 \vec{S}_1 \cdot \vec{S}_1 + \frac{4}{7} \vec{S}_1 \cdot \vec{v}_1 \vec{S}_1 \cdot \vec{v}_2 + \frac{2}{7} \vec{S}_1 \cdot \vec{S}_1 \vec{v}_1 \cdot \vec{v}_1 + \frac{2}{7} \vec{S}_1 \cdot \vec{S}_1 \vec{v}_1 \cdot \vec{v}_2 \right) \Big) \Big) \Big) C_{ES^2_1} \Big\}
\end{aligned}$$

{DiagS1CES2[3, 1, 32],

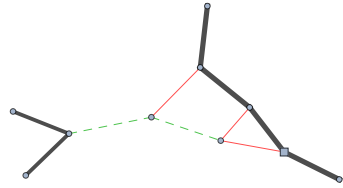

$$\begin{aligned}
& G^3 m_1 m_2 \left( \frac{10 \hat{n} \cdot \vec{S}_1 \hat{n} \cdot \vec{S}_1 \hat{n} \cdot \vec{v}_2 - \frac{98}{25} \vec{S}_1 \cdot \vec{S}_1 \hat{n} \cdot \vec{v}_2 + \frac{2}{25} \hat{n} \cdot \vec{S}_1 \vec{S}_1 \cdot \vec{v}_2 + \frac{2}{25} \hat{n} \cdot \vec{S}_1 \vec{S}_1 \cdot \vec{v}_2}{r^4} + \right. \\
& \quad \frac{1}{r^5} \left( -\frac{167}{4} \hat{n} \cdot \vec{v}_1 \hat{n} \cdot \vec{v}_2 (\hat{n} \cdot \vec{S}_1)^2 + \frac{261}{196} \vec{v}_1 \cdot \vec{v}_2 (\hat{n} \cdot \vec{S}_1)^2 + \frac{1045}{98} \hat{n} \cdot \vec{v}_2 \vec{S}_1 \cdot \vec{v}_1 \hat{n} \cdot \vec{S}_1 + \right. \\
& \quad \frac{765}{98} \hat{n} \cdot \vec{v}_1 \vec{S}_1 \cdot \vec{v}_2 \hat{n} \cdot \vec{S}_1 + \frac{1801}{196} \hat{n} \cdot \vec{v}_1 \hat{n} \cdot \vec{v}_2 \vec{S}_1 \cdot \vec{S}_1 - \frac{69}{98} \vec{S}_1 \cdot \vec{v}_1 \vec{S}_1 \cdot \vec{v}_2 - \frac{97}{196} \vec{S}_1 \cdot \vec{S}_1 \vec{v}_1 \cdot \vec{v}_2 \Big) + \\
& \quad \left( \frac{-12 \hat{n} \cdot \vec{S}_1 \hat{n} \cdot \vec{S}_1 \hat{n} \cdot \vec{v}_2 + \frac{12}{5} \vec{S}_1 \cdot \vec{S}_1 \hat{n} \cdot \vec{v}_2 + \frac{12}{5} \hat{n} \cdot \vec{S}_1 \vec{S}_1 \cdot \vec{v}_2 + \frac{12}{5} \hat{n} \cdot \vec{S}_1 \vec{S}_1 \cdot \vec{v}_2}{r^4} + \frac{1}{r^5} \right. \\
& \quad \left. \left( 45 \hat{n} \cdot \vec{v}_1 \hat{n} \cdot \vec{v}_2 (\hat{n} \cdot \vec{S}_1)^2 - \frac{45}{7} \vec{v}_1 \cdot \vec{v}_2 (\hat{n} \cdot \vec{S}_1)^2 - \frac{90}{7} \hat{n} \cdot \vec{v}_2 \vec{S}_1 \cdot \vec{v}_1 \hat{n} \cdot \vec{S}_1 - \frac{90}{7} \hat{n} \cdot \vec{v}_1 \vec{S}_1 \cdot \vec{v}_2 \hat{n} \cdot \vec{S}_1 - \right. \right.
\end{aligned}$$

$$\begin{aligned}
& \left. \left( \frac{45}{7} \hat{n} \cdot \vec{v}_1 \hat{n} \cdot \vec{v}_2 \vec{S}_1 \cdot \vec{S}_1 + \frac{18}{7} \vec{S}_1 \cdot \vec{v}_1 \vec{S}_1 \cdot \vec{v}_2 + \frac{9}{7} \vec{S}_1 \cdot \vec{S}_1 \vec{v}_1 \cdot \vec{v}_2 \right) \log \left( \frac{r}{R_\theta} \right) + \right. \\
& \frac{1}{\epsilon_d} \left( \frac{4 \hat{n} \cdot \vec{S}_1 \hat{n} \cdot \vec{S}_1 \hat{n} \cdot \vec{v}_2 - \frac{4}{5} \vec{S}_1 \cdot \vec{S}_1 \hat{n} \cdot \vec{v}_2 - \frac{4}{5} \hat{n} \cdot \vec{S}_1 \vec{S}_1 \cdot \vec{v}_2 - \frac{4}{5} \hat{n} \cdot \vec{S}_1 \vec{S}_1 \cdot \vec{v}_2}{r^4} + \frac{1}{r^5} \right. \\
& \left( -15 \hat{n} \cdot \vec{v}_1 \hat{n} \cdot \vec{v}_2 (\hat{n} \cdot \vec{S}_1)^2 + \frac{15}{7} \vec{v}_1 \cdot \vec{v}_2 (\hat{n} \cdot \vec{S}_1)^2 + \frac{30}{7} \hat{n} \cdot \vec{v}_2 \vec{S}_1 \cdot \vec{v}_1 \hat{n} \cdot \vec{S}_1 + \right. \\
& \left. \left. \frac{30}{7} \hat{n} \cdot \vec{v}_1 \vec{S}_1 \cdot \vec{v}_2 \hat{n} \cdot \vec{S}_1 + \frac{15}{7} \hat{n} \cdot \vec{v}_1 \hat{n} \cdot \vec{v}_2 \vec{S}_1 \cdot \vec{S}_1 - \frac{6}{7} \vec{S}_1 \cdot \vec{v}_1 \vec{S}_1 \cdot \vec{v}_2 - \frac{3}{7} \vec{S}_1 \cdot \vec{S}_1 \vec{v}_1 \cdot \vec{v}_2 \right) \right) \Bigg\} c_{\text{ES}^2 1}
\end{aligned}$$

{DiagS1CES2[3, 1, 33],

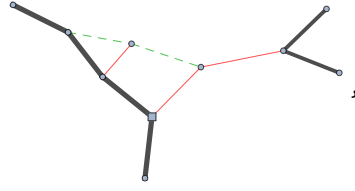

$$\begin{aligned}
& G^3 m_1 m_2 \left( \frac{-22 \hat{n} \cdot \vec{S}_1 \hat{n} \cdot \vec{S}_1 \hat{n} \cdot \vec{v}_1 + \frac{174}{25} \vec{S}_1 \cdot \vec{S}_1 \hat{n} \cdot \vec{v}_1 + \frac{74}{25} \hat{n} \cdot \vec{S}_1 \vec{S}_1 \cdot \vec{v}_1 + \frac{74}{25} \hat{n} \cdot \vec{S}_1 \vec{S}_1 \cdot \vec{v}_1}{r^4} + \frac{1}{r^5} \right. \\
& \left( 61 (\hat{n} \cdot \vec{v}_1)^2 (\hat{n} \cdot \vec{S}_1)^2 + 61 \hat{n} \cdot \vec{v}_1 \hat{n} \cdot \vec{v}_2 (\hat{n} \cdot \vec{S}_1)^2 - \frac{337}{49} \vec{v}_1 \cdot \vec{v}_1 (\hat{n} \cdot \vec{S}_1)^2 - \frac{337}{49} \vec{v}_1 \cdot \vec{v}_2 (\hat{n} \cdot \vec{S}_1)^2 - \right. \\
& \frac{1516}{49} \hat{n} \cdot \vec{v}_1 \vec{S}_1 \cdot \vec{v}_1 \hat{n} \cdot \vec{S}_1 - \frac{842}{49} \hat{n} \cdot \vec{v}_2 \vec{S}_1 \cdot \vec{v}_1 \hat{n} \cdot \vec{S}_1 - \frac{674}{49} \hat{n} \cdot \vec{v}_1 \vec{S}_1 \cdot \vec{v}_2 \hat{n} \cdot \vec{S}_1 + \frac{118}{49} (\vec{S}_1 \cdot \vec{v}_1)^2 - \\
& \frac{631}{49} (\hat{n} \cdot \vec{v}_1)^2 \vec{S}_1 \cdot \vec{S}_1 - \frac{631}{49} \hat{n} \cdot \vec{v}_1 \hat{n} \cdot \vec{v}_2 \vec{S}_1 \cdot \vec{S}_1 + \frac{118}{49} \vec{S}_1 \cdot \vec{v}_1 \vec{S}_1 \cdot \vec{v}_2 + \frac{101}{49} \vec{S}_1 \cdot \vec{S}_1 \vec{v}_1 \cdot \vec{v}_1 + \frac{101}{49} \vec{S}_1 \cdot \vec{S}_1 \vec{v}_1 \cdot \vec{v}_2 \Big) + \\
& \left( \frac{36 \hat{n} \cdot \vec{S}_1 \hat{n} \cdot \vec{S}_1 \hat{n} \cdot \vec{v}_1 - \frac{36}{5} \vec{S}_1 \cdot \vec{S}_1 \hat{n} \cdot \vec{v}_1 - \frac{36}{5} \hat{n} \cdot \vec{S}_1 \vec{S}_1 \cdot \vec{v}_1 - \frac{36}{5} \hat{n} \cdot \vec{S}_1 \vec{S}_1 \cdot \vec{v}_1}{r^4} + \frac{1}{r^5} \right. \\
& \left( -90 (\hat{n} \cdot \vec{v}_1)^2 (\hat{n} \cdot \vec{S}_1)^2 - 90 \hat{n} \cdot \vec{v}_1 \hat{n} \cdot \vec{v}_2 (\hat{n} \cdot \vec{S}_1)^2 + \frac{90}{7} \vec{v}_1 \cdot \vec{v}_1 (\hat{n} \cdot \vec{S}_1)^2 + \frac{90}{7} \vec{v}_1 \cdot \vec{v}_2 (\hat{n} \cdot \vec{S}_1)^2 + \right. \\
& \frac{360}{7} \hat{n} \cdot \vec{v}_1 \vec{S}_1 \cdot \vec{v}_1 \hat{n} \cdot \vec{S}_1 + \frac{180}{7} \hat{n} \cdot \vec{v}_2 \vec{S}_1 \cdot \vec{v}_1 \hat{n} \cdot \vec{S}_1 + \frac{180}{7} \hat{n} \cdot \vec{v}_1 \vec{S}_1 \cdot \vec{v}_2 \hat{n} \cdot \vec{S}_1 - \frac{36}{7} (\vec{S}_1 \cdot \vec{v}_1)^2 + \\
& \left. \left. \frac{90}{7} (\hat{n} \cdot \vec{v}_1)^2 \vec{S}_1 \cdot \vec{S}_1 + \frac{90}{7} \hat{n} \cdot \vec{v}_1 \hat{n} \cdot \vec{v}_2 \vec{S}_1 \cdot \vec{S}_1 - \frac{36}{7} \vec{S}_1 \cdot \vec{v}_1 \vec{S}_1 \cdot \vec{v}_2 - \frac{18}{7} \vec{S}_1 \cdot \vec{S}_1 \vec{v}_1 \cdot \vec{v}_1 - \frac{18}{7} \vec{S}_1 \cdot \vec{S}_1 \vec{v}_1 \cdot \vec{v}_2 \right) \right) \\
& \log \left( \frac{r}{R_\theta} \right) + \frac{1}{\epsilon_d} \left( \frac{-12 \hat{n} \cdot \vec{S}_1 \hat{n} \cdot \vec{S}_1 \hat{n} \cdot \vec{v}_1 + \frac{12}{5} \vec{S}_1 \cdot \vec{S}_1 \hat{n} \cdot \vec{v}_1 + \frac{12}{5} \hat{n} \cdot \vec{S}_1 \vec{S}_1 \cdot \vec{v}_1 + \frac{12}{5} \hat{n} \cdot \vec{S}_1 \vec{S}_1 \cdot \vec{v}_1}{r^4} + \frac{1}{r^5} \right. \\
& \left( 30 (\hat{n} \cdot \vec{v}_1)^2 (\hat{n} \cdot \vec{S}_1)^2 + 30 \hat{n} \cdot \vec{v}_1 \hat{n} \cdot \vec{v}_2 (\hat{n} \cdot \vec{S}_1)^2 - \frac{30}{7} \vec{v}_1 \cdot \vec{v}_1 (\hat{n} \cdot \vec{S}_1)^2 - \frac{30}{7} \vec{v}_1 \cdot \vec{v}_2 (\hat{n} \cdot \vec{S}_1)^2 - \right. \\
& \frac{120}{7} \hat{n} \cdot \vec{v}_1 \vec{S}_1 \cdot \vec{v}_1 \hat{n} \cdot \vec{S}_1 - \frac{60}{7} \hat{n} \cdot \vec{v}_2 \vec{S}_1 \cdot \vec{v}_1 \hat{n} \cdot \vec{S}_1 - \frac{60}{7} \hat{n} \cdot \vec{v}_1 \vec{S}_1 \cdot \vec{v}_2 \hat{n} \cdot \vec{S}_1 + \frac{12}{7} (\vec{S}_1 \cdot \vec{v}_1)^2 - \\
& \left. \left. \frac{30}{7} (\hat{n} \cdot \vec{v}_1)^2 \vec{S}_1 \cdot \vec{S}_1 - \frac{30}{7} \hat{n} \cdot \vec{v}_1 \hat{n} \cdot \vec{v}_2 \vec{S}_1 \cdot \vec{S}_1 + \frac{12}{7} \vec{S}_1 \cdot \vec{v}_1 \vec{S}_1 \cdot \vec{v}_2 + \frac{6}{7} \vec{S}_1 \cdot \vec{S}_1 \vec{v}_1 \cdot \vec{v}_1 + \frac{6}{7} \vec{S}_1 \cdot \vec{S}_1 \vec{v}_1 \cdot \vec{v}_2 \right) \right) \Bigg\} c_{\text{ES}^2 1}
\end{aligned}$$



$\{\text{DiagS1CES2}[3, 1, 34],$ 
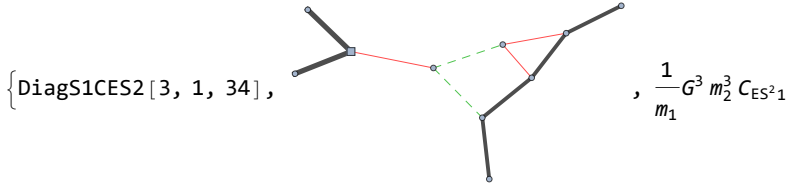
 $, \frac{1}{m_1} G^3 m_2^3 C_{\text{ES}^2 1}$

$$\left( \frac{7 \left( \hat{n} \cdot \vec{S}_1 \right)^2 \left( \hat{n} \cdot \vec{v}_2 \right)^2 - \vec{v}_2 \cdot \vec{v}_2 \left( \hat{n} \cdot \vec{S}_1 \right)^2 - 4 \hat{n} \cdot \vec{S}_1 \hat{n} \cdot \vec{v}_2 \vec{S}_1 \cdot \vec{v}_2 - \vec{S}_1 \cdot \vec{S}_1 \left( \hat{n} \cdot \vec{v}_2 \right)^2 + \frac{2}{5} \left( \vec{S}_1 \cdot \vec{v}_2 \right)^2 + \frac{1}{5} \vec{S}_1 \cdot \vec{S}_1 \vec{v}_2 \cdot \vec{v}_2}{r^5 \in_d} + \right.$$

$$\frac{1}{r^5} \log \left( \frac{r}{R_0} \right) \left( -21 \left( \hat{n} \cdot \vec{S}_1 \right)^2 \left( \hat{n} \cdot \vec{v}_2 \right)^2 + 3 \vec{v}_2 \cdot \vec{v}_2 \left( \hat{n} \cdot \vec{S}_1 \right)^2 + 12 \hat{n} \cdot \vec{S}_1 \hat{n} \cdot \vec{v}_2 \vec{S}_1 \cdot \vec{v}_2 + \right.$$

$$3 \vec{S}_1 \cdot \vec{S}_1 \left( \hat{n} \cdot \vec{v}_2 \right)^2 - \frac{6}{5} \left( \vec{S}_1 \cdot \vec{v}_2 \right)^2 - \frac{3}{5} \vec{S}_1 \cdot \vec{S}_1 \vec{v}_2 \cdot \vec{v}_2 \Big) + \frac{1}{r^5} \left( 24 \left( \hat{n} \cdot \vec{S}_1 \right)^2 \left( \hat{n} \cdot \vec{v}_2 \right)^2 + \right.$$

$$\left. \left. 3 \vec{v}_2 \cdot \vec{v}_2 \left( \hat{n} \cdot \vec{S}_1 \right)^2 - 12 \hat{n} \cdot \vec{S}_1 \hat{n} \cdot \vec{v}_2 \vec{S}_1 \cdot \vec{v}_2 - 6 \vec{S}_1 \cdot \vec{S}_1 \left( \hat{n} \cdot \vec{v}_2 \right)^2 + \frac{24}{25} \left( \vec{S}_1 \cdot \vec{v}_2 \right)^2 - \frac{63}{25} \vec{S}_1 \cdot \vec{S}_1 \vec{v}_2 \cdot \vec{v}_2 \right) \right) \Bigg\}$$

$\{\text{DiagS1CES2}[3, 1, 35],$ 
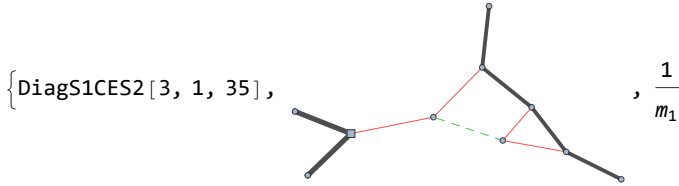
 $, \frac{1}{m_1}$

$$G^3 m_2^3 C_{\text{ES}^2 1} \left( \frac{1}{r^5 \in_d} \left( -\frac{21}{4} \left( \hat{n} \cdot \vec{S}_1 \right)^2 \left( \hat{n} \cdot \vec{v}_2 \right)^2 + \frac{3}{4} \vec{v}_2 \cdot \vec{v}_2 \left( \hat{n} \cdot \vec{S}_1 \right)^2 + 3 \hat{n} \cdot \vec{S}_1 \hat{n} \cdot \vec{v}_2 \vec{S}_1 \cdot \vec{v}_2 + \right. \right.$$

$$\frac{3}{4} \vec{S}_1 \cdot \vec{S}_1 \left( \hat{n} \cdot \vec{v}_2 \right)^2 - \frac{3}{10} \left( \vec{S}_1 \cdot \vec{v}_2 \right)^2 - \frac{3}{20} \vec{S}_1 \cdot \vec{S}_1 \vec{v}_2 \cdot \vec{v}_2 \Big) + \frac{1}{r^5} \log \left( \frac{r}{R_0} \right) \left( \frac{63}{4} \left( \hat{n} \cdot \vec{S}_1 \right)^2 \left( \hat{n} \cdot \vec{v}_2 \right)^2 - \right.$$

$$\frac{9}{4} \vec{v}_2 \cdot \vec{v}_2 \left( \hat{n} \cdot \vec{S}_1 \right)^2 - 9 \hat{n} \cdot \vec{S}_1 \hat{n} \cdot \vec{v}_2 \vec{S}_1 \cdot \vec{v}_2 - \frac{9}{4} \vec{S}_1 \cdot \vec{S}_1 \left( \hat{n} \cdot \vec{v}_2 \right)^2 + \frac{9}{10} \left( \vec{S}_1 \cdot \vec{v}_2 \right)^2 + \frac{9}{20} \vec{S}_1 \cdot \vec{S}_1 \vec{v}_2 \cdot \vec{v}_2 \Big) +$$

$$\frac{1}{r^5} \left( -\frac{81}{8} \left( \hat{n} \cdot \vec{S}_1 \right)^2 \left( \hat{n} \cdot \vec{v}_2 \right)^2 + \frac{35}{2} \left( \hat{n} \cdot \vec{S}_1 \right)^2 \hat{n} \cdot \vec{v}_1 \hat{n} \cdot \vec{v}_2 - \frac{5}{2} \vec{v}_1 \cdot \vec{v}_2 \left( \hat{n} \cdot \vec{S}_1 \right)^2 + \frac{13}{8} \vec{v}_2 \cdot \vec{v}_2 \left( \hat{n} \cdot \vec{S}_1 \right)^2 - \right.$$

$$5 \hat{n} \cdot \vec{S}_1 \hat{n} \cdot \vec{v}_2 \vec{S}_1 \cdot \vec{v}_1 - 5 \hat{n} \cdot \vec{S}_1 \hat{n} \cdot \vec{v}_1 \vec{S}_1 \cdot \vec{v}_2 + \frac{9}{2} \hat{n} \cdot \vec{S}_1 \hat{n} \cdot \vec{v}_2 \vec{S}_1 \cdot \vec{v}_2 + \frac{27}{8} \vec{S}_1 \cdot \vec{S}_1 \left( \hat{n} \cdot \vec{v}_2 \right)^2 -$$

$$\frac{5}{2} \vec{S}_1 \cdot \vec{S}_1 \hat{n} \cdot \vec{v}_1 \hat{n} \cdot \vec{v}_2 - \frac{27}{100} \left( \vec{S}_1 \cdot \vec{v}_2 \right)^2 + \vec{S}_1 \cdot \vec{v}_1 \vec{S}_1 \cdot \vec{v}_2 + \frac{1}{2} \vec{S}_1 \cdot \vec{S}_1 \vec{v}_1 \cdot \vec{v}_2 - \frac{177}{200} \vec{S}_1 \cdot \vec{S}_1 \vec{v}_2 \cdot \vec{v}_2 \Big) +$$

$$\left. \frac{-5 \hat{n} \cdot \vec{S}_1 \hat{n} \cdot \vec{S}_1 \hat{n} \cdot \vec{v}_2 + \vec{S}_1 \cdot \vec{S}_1 \hat{n} \cdot \vec{v}_2 + \hat{n} \cdot \vec{S}_1 \vec{S}_1 \cdot \vec{v}_2 + \hat{n} \cdot \vec{S}_1 \vec{S}_1 \cdot \vec{v}_2}{r^4} \right) \Bigg\}$$

$\{\text{DiagS1CES2}[3, 1, 36],$ 
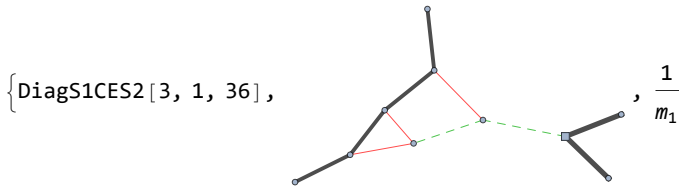
 $, \frac{1}{m_1}$

$$G^3 m_2^3 \left( \frac{26 \hat{n} \cdot \vec{S}_1 \hat{n} \cdot \vec{S}_1 \hat{n} \cdot \vec{v}_2 - 14 \vec{S}_1 \cdot \vec{S}_1 \hat{n} \cdot \vec{v}_2 - 2 \hat{n} \cdot \vec{S}_1 \vec{S}_1 \cdot \vec{v}_2 - 2 \hat{n} \cdot \vec{S}_1 \vec{S}_1 \cdot \vec{v}_2}{r^4} + \right.$$

$$\frac{1}{r^5} \left( -106 \hat{n} \cdot \vec{v}_1 \hat{n} \cdot \vec{v}_2 \left( \hat{n} \cdot \vec{S}_1 \right)^2 + 3 \vec{v}_1 \cdot \vec{v}_2 \left( \hat{n} \cdot \vec{S}_1 \right)^2 + 26 \hat{n} \cdot \vec{v}_2 \vec{S}_1 \cdot \vec{v}_1 \hat{n} \cdot \vec{S}_1 + \right.$$

$$\begin{aligned}
& 26 \hat{n} \cdot \vec{v}_1 \vec{S}_1 \cdot \vec{v}_2 \hat{n} \cdot \vec{S}_1 + 28 \hat{n} \cdot \vec{v}_1 \hat{n} \cdot \vec{v}_2 \vec{S}_1 \cdot \vec{S}_1 - 4 \vec{S}_1 \cdot \vec{v}_1 \vec{S}_1 \cdot \vec{v}_2 + \vec{S}_1 \cdot \vec{S}_1 \vec{v}_1 \cdot \vec{v}_2 \Big) + \\
& \left( \frac{-30 \hat{n} \cdot \vec{S}_1 \hat{n} \cdot \vec{S}_1 \hat{n} \cdot \vec{v}_2 + 6 \vec{S}_1 \cdot \vec{S}_1 \hat{n} \cdot \vec{v}_2 + 6 \hat{n} \cdot \vec{S}_1 \vec{S}_1 \cdot \vec{v}_2 + 6 \hat{n} \cdot \vec{S}_1 \vec{S}_1 \cdot \vec{v}_2}{r^4} + \frac{1}{r^5} \right. \\
& \left( 105 \hat{n} \cdot \vec{v}_1 \hat{n} \cdot \vec{v}_2 \left( \hat{n} \cdot \vec{S}_1 \right)^2 - 15 \vec{v}_1 \cdot \vec{v}_2 \left( \hat{n} \cdot \vec{S}_1 \right)^2 - 30 \hat{n} \cdot \vec{v}_2 \vec{S}_1 \cdot \vec{v}_1 \hat{n} \cdot \vec{S}_1 - \right. \\
& \left. 30 \hat{n} \cdot \vec{v}_1 \vec{S}_1 \cdot \vec{v}_2 \hat{n} \cdot \vec{S}_1 - 15 \hat{n} \cdot \vec{v}_1 \hat{n} \cdot \vec{v}_2 \vec{S}_1 \cdot \vec{S}_1 + 6 \vec{S}_1 \cdot \vec{v}_1 \vec{S}_1 \cdot \vec{v}_2 + 3 \vec{S}_1 \cdot \vec{S}_1 \vec{v}_1 \cdot \vec{v}_2 \right) \log \left( \frac{r}{R_0} \right) + \\
& \frac{1}{\epsilon_d} \left( \frac{10 \hat{n} \cdot \vec{S}_1 \hat{n} \cdot \vec{S}_1 \hat{n} \cdot \vec{v}_2 - 2 \vec{S}_1 \cdot \vec{S}_1 \hat{n} \cdot \vec{v}_2 - 2 \hat{n} \cdot \vec{S}_1 \vec{S}_1 \cdot \vec{v}_2 - 2 \hat{n} \cdot \vec{S}_1 \vec{S}_1 \cdot \vec{v}_2}{r^4} + \frac{1}{r^5} \right. \\
& \left( -35 \hat{n} \cdot \vec{v}_1 \hat{n} \cdot \vec{v}_2 \left( \hat{n} \cdot \vec{S}_1 \right)^2 + 5 \vec{v}_1 \cdot \vec{v}_2 \left( \hat{n} \cdot \vec{S}_1 \right)^2 + 10 \hat{n} \cdot \vec{v}_2 \vec{S}_1 \cdot \vec{v}_1 \hat{n} \cdot \vec{S}_1 + \right. \\
& \left. 10 \hat{n} \cdot \vec{v}_1 \vec{S}_1 \cdot \vec{v}_2 \hat{n} \cdot \vec{S}_1 + 5 \hat{n} \cdot \vec{v}_1 \hat{n} \cdot \vec{v}_2 \vec{S}_1 \cdot \vec{S}_1 - 2 \vec{S}_1 \cdot \vec{v}_1 \vec{S}_1 \cdot \vec{v}_2 - \vec{S}_1 \cdot \vec{S}_1 \vec{v}_1 \cdot \vec{v}_2 \right) \Big) \Bigg\} C_{ES^2 1} \Bigg\}
\end{aligned}$$

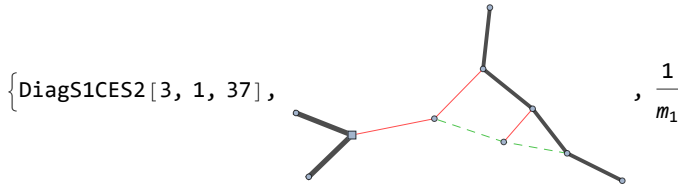

$$\begin{aligned}
& G^3 m_2^3 \left( \frac{-42 \hat{n} \cdot \vec{S}_1 \hat{n} \cdot \vec{S}_1 \hat{n} \cdot \vec{v}_2 + 18 \vec{S}_1 \cdot \vec{S}_1 \hat{n} \cdot \vec{v}_2 + 6 \hat{n} \cdot \vec{S}_1 \vec{S}_1 \cdot \vec{v}_2 + 6 \hat{n} \cdot \vec{S}_1 \vec{S}_1 \cdot \vec{v}_2}{r^4} + \frac{1}{r^5} \right. \\
& \left( 177 \left( \hat{n} \cdot \vec{v}_2 \right)^2 \left( \hat{n} \cdot \vec{S}_1 \right)^2 + 177 \hat{n} \cdot \vec{v}_1 \hat{n} \cdot \vec{v}_2 \left( \hat{n} \cdot \vec{S}_1 \right)^2 - 21 \vec{v}_1 \cdot \vec{v}_2 \left( \hat{n} \cdot \vec{S}_1 \right)^2 - 21 \vec{v}_2 \cdot \vec{v}_2 \left( \hat{n} \cdot \vec{S}_1 \right)^2 - \right. \\
& 42 \hat{n} \cdot \vec{v}_2 \vec{S}_1 \cdot \vec{v}_1 \hat{n} \cdot \vec{S}_1 - 42 \hat{n} \cdot \vec{v}_1 \vec{S}_1 \cdot \vec{v}_2 \hat{n} \cdot \vec{S}_1 - 84 \hat{n} \cdot \vec{v}_2 \vec{S}_1 \cdot \vec{v}_2 \hat{n} \cdot \vec{S}_1 + 6 \left( \vec{S}_1 \cdot \vec{v}_2 \right)^2 - \\
& 51 \left( \hat{n} \cdot \vec{v}_2 \right)^2 \vec{S}_1 \cdot \vec{S}_1 - 51 \hat{n} \cdot \vec{v}_1 \hat{n} \cdot \vec{v}_2 \vec{S}_1 \cdot \vec{S}_1 + 6 \vec{S}_1 \cdot \vec{v}_1 \vec{S}_1 \cdot \vec{v}_2 + 9 \vec{S}_1 \cdot \vec{S}_1 \vec{v}_1 \cdot \vec{v}_2 + 9 \vec{S}_1 \cdot \vec{S}_1 \vec{v}_2 \cdot \vec{v}_2 \Big) + \\
& \left( \frac{60 \hat{n} \cdot \vec{S}_1 \hat{n} \cdot \vec{S}_1 \hat{n} \cdot \vec{v}_2 - 12 \vec{S}_1 \cdot \vec{S}_1 \hat{n} \cdot \vec{v}_2 - 12 \hat{n} \cdot \vec{S}_1 \vec{S}_1 \cdot \vec{v}_2 - 12 \hat{n} \cdot \vec{S}_1 \vec{S}_1 \cdot \vec{v}_2}{r^4} + \frac{1}{r^5} \right. \\
& \left( -210 \left( \hat{n} \cdot \vec{v}_2 \right)^2 \left( \hat{n} \cdot \vec{S}_1 \right)^2 - 210 \hat{n} \cdot \vec{v}_1 \hat{n} \cdot \vec{v}_2 \left( \hat{n} \cdot \vec{S}_1 \right)^2 + 30 \vec{v}_1 \cdot \vec{v}_2 \left( \hat{n} \cdot \vec{S}_1 \right)^2 + 30 \vec{v}_2 \cdot \vec{v}_2 \left( \hat{n} \cdot \vec{S}_1 \right)^2 + \right. \\
& 60 \hat{n} \cdot \vec{v}_2 \vec{S}_1 \cdot \vec{v}_1 \hat{n} \cdot \vec{S}_1 + 60 \hat{n} \cdot \vec{v}_1 \vec{S}_1 \cdot \vec{v}_2 \hat{n} \cdot \vec{S}_1 + 120 \hat{n} \cdot \vec{v}_2 \vec{S}_1 \cdot \vec{v}_2 \hat{n} \cdot \vec{S}_1 - 12 \left( \vec{S}_1 \cdot \vec{v}_2 \right)^2 + 30 \left( \hat{n} \cdot \vec{v}_2 \right)^2 \vec{S}_1 \cdot \vec{S}_1 + \\
& 30 \hat{n} \cdot \vec{v}_1 \hat{n} \cdot \vec{v}_2 \vec{S}_1 \cdot \vec{S}_1 - 12 \vec{S}_1 \cdot \vec{v}_1 \vec{S}_1 \cdot \vec{v}_2 - 6 \vec{S}_1 \cdot \vec{S}_1 \vec{v}_1 \cdot \vec{v}_2 - 6 \vec{S}_1 \cdot \vec{S}_1 \vec{v}_2 \cdot \vec{v}_2 \Big) \log \left( \frac{r}{R_0} \right) + \\
& \frac{1}{\epsilon_d} \left( \frac{-20 \hat{n} \cdot \vec{S}_1 \hat{n} \cdot \vec{S}_1 \hat{n} \cdot \vec{v}_2 + 4 \vec{S}_1 \cdot \vec{S}_1 \hat{n} \cdot \vec{v}_2 + 4 \hat{n} \cdot \vec{S}_1 \vec{S}_1 \cdot \vec{v}_2 + 4 \hat{n} \cdot \vec{S}_1 \vec{S}_1 \cdot \vec{v}_2}{r^4} + \frac{1}{r^5} \right. \\
& \left( 70 \left( \hat{n} \cdot \vec{v}_2 \right)^2 \left( \hat{n} \cdot \vec{S}_1 \right)^2 + 70 \hat{n} \cdot \vec{v}_1 \hat{n} \cdot \vec{v}_2 \left( \hat{n} \cdot \vec{S}_1 \right)^2 - 10 \vec{v}_1 \cdot \vec{v}_2 \left( \hat{n} \cdot \vec{S}_1 \right)^2 - 10 \vec{v}_2 \cdot \vec{v}_2 \left( \hat{n} \cdot \vec{S}_1 \right)^2 - \right. \\
& 20 \hat{n} \cdot \vec{v}_2 \vec{S}_1 \cdot \vec{v}_1 \hat{n} \cdot \vec{S}_1 - 20 \hat{n} \cdot \vec{v}_1 \vec{S}_1 \cdot \vec{v}_2 \hat{n} \cdot \vec{S}_1 - 40 \hat{n} \cdot \vec{v}_2 \vec{S}_1 \cdot \vec{v}_2 \hat{n} \cdot \vec{S}_1 + 4 \left( \vec{S}_1 \cdot \vec{v}_2 \right)^2 - \\
& 10 \left( \hat{n} \cdot \vec{v}_2 \right)^2 \vec{S}_1 \cdot \vec{S}_1 - 10 \hat{n} \cdot \vec{v}_1 \hat{n} \cdot \vec{v}_2 \vec{S}_1 \cdot \vec{S}_1 + 4 \vec{S}_1 \cdot \vec{v}_1 \vec{S}_1 \cdot \vec{v}_2 + 2 \vec{S}_1 \cdot \vec{S}_1 \vec{v}_1 \cdot \vec{v}_2 + 2 \vec{S}_1 \cdot \vec{S}_1 \vec{v}_2 \cdot \vec{v}_2 \Big) \Bigg\} C_{ES^2 1} \Bigg\}
\end{aligned}$$

{DiagS1CES2[3, 1, 38],

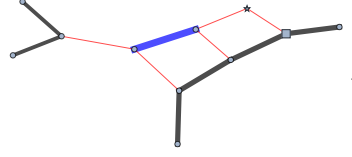

,

$$\begin{aligned}
 & G^3 m_1 m_2 \left( \frac{1}{r^4} \left( \frac{20}{147} \hat{n} \cdot \vec{S}_1 \hat{n} \cdot \vec{S}_1 \hat{n} \cdot \vec{v}_1 + \frac{3092 \vec{S}_1 \cdot \vec{S}_1 \hat{n} \cdot \vec{v}_1}{3675} - \hat{n} \cdot \vec{S}_1 \hat{n} \cdot \vec{S}_1 \hat{n} \cdot \vec{v}_2 + \right. \right. \\
 & \quad \left. \frac{572 \hat{n} \cdot \vec{S}_1 \vec{S}_1 \cdot \vec{v}_1}{3675} + \frac{2}{25} \hat{n} \cdot \vec{S}_1 \vec{S}_1 \cdot \vec{v}_2 - \frac{23}{25} \hat{n} \cdot \vec{v}_2 \vec{S}_1 \cdot \vec{S}_1 + \frac{572 \hat{n} \cdot \vec{S}_1 \vec{S}_1 \cdot \vec{v}_1}{3675} + \frac{2}{25} \hat{n} \cdot \vec{S}_1 \vec{S}_1 \cdot \vec{v}_2 \right) + \frac{1}{r^5} \\
 & \quad \left( -\frac{17}{12} (\hat{n} \cdot \vec{v}_1)^2 (\hat{n} \cdot \vec{S}_1)^2 + \frac{11}{3} \hat{n} \cdot \vec{v}_1 \hat{n} \cdot \vec{v}_2 (\hat{n} \cdot \vec{S}_1)^2 + \frac{13}{196} \vec{v}_1 \cdot \vec{v}_1 (\hat{n} \cdot \vec{S}_1)^2 - \frac{127}{294} \vec{v}_1 \cdot \vec{v}_2 (\hat{n} \cdot \vec{S}_1)^2 + \right. \\
 & \quad \frac{41}{49} \hat{n} \cdot \vec{v}_1 \vec{S}_1 \cdot \vec{v}_1 \hat{n} \cdot \vec{S}_1 - \frac{211}{147} \hat{n} \cdot \vec{v}_2 \vec{S}_1 \cdot \vec{v}_1 \hat{n} \cdot \vec{S}_1 - \frac{127}{147} \hat{n} \cdot \vec{v}_1 \vec{S}_1 \cdot \vec{v}_2 \hat{n} \cdot \vec{S}_1 - \frac{307 (\vec{S}_1 \cdot \vec{v}_1)^2}{7350} - \\
 & \quad \left. \frac{73}{588} (\hat{n} \cdot \vec{v}_1)^2 \vec{S}_1 \cdot \vec{S}_1 + \frac{10}{147} \hat{n} \cdot \vec{v}_1 \hat{n} \cdot \vec{v}_2 \vec{S}_1 \cdot \vec{S}_1 + \frac{866 \vec{S}_1 \cdot \vec{v}_1 \vec{S}_1 \cdot \vec{v}_2}{3675} + \frac{253 \vec{S}_1 \cdot \vec{S}_1 \vec{v}_1 \cdot \vec{v}_1}{14700} - \frac{289 \vec{S}_1 \cdot \vec{S}_1 \vec{v}_1 \cdot \vec{v}_2}{7350} \right) + \\
 & \quad \left( \frac{1}{r^4} \left( -\frac{12}{7} \hat{n} \cdot \vec{S}_1 \hat{n} \cdot \vec{S}_1 \hat{n} \cdot \vec{v}_1 + \frac{12}{35} \vec{S}_1 \cdot \vec{S}_1 \hat{n} \cdot \vec{v}_1 + 3 \hat{n} \cdot \vec{S}_1 \hat{n} \cdot \vec{S}_1 \hat{n} \cdot \vec{v}_2 + \frac{12}{35} \hat{n} \cdot \vec{S}_1 \vec{S}_1 \cdot \vec{v}_1 - \right. \right. \\
 & \quad \left. \frac{3}{5} \hat{n} \cdot \vec{S}_1 \vec{S}_1 \cdot \vec{v}_2 - \frac{3}{5} \hat{n} \cdot \vec{v}_2 \vec{S}_1 \cdot \vec{S}_1 + \frac{12}{35} \hat{n} \cdot \vec{S}_1 \vec{S}_1 \cdot \vec{v}_1 - \frac{3}{5} \hat{n} \cdot \vec{S}_1 \vec{S}_1 \cdot \vec{v}_2 \right) + \frac{1}{r^5} \\
 & \quad \left( 2 (\hat{n} \cdot \vec{v}_1)^2 (\hat{n} \cdot \vec{S}_1)^2 - \frac{9}{2} \hat{n} \cdot \vec{v}_1 \hat{n} \cdot \vec{v}_2 (\hat{n} \cdot \vec{S}_1)^2 - \frac{2}{7} \vec{v}_1 \cdot \vec{v}_1 (\hat{n} \cdot \vec{S}_1)^2 + \frac{9}{14} \vec{v}_1 \cdot \vec{v}_2 (\hat{n} \cdot \vec{S}_1)^2 - \right. \\
 & \quad \frac{8}{7} \hat{n} \cdot \vec{v}_1 \vec{S}_1 \cdot \vec{v}_1 \hat{n} \cdot \vec{S}_1 + \frac{9}{7} \hat{n} \cdot \vec{v}_2 \vec{S}_1 \cdot \vec{v}_1 \hat{n} \cdot \vec{S}_1 + \frac{9}{7} \hat{n} \cdot \vec{v}_1 \vec{S}_1 \cdot \vec{v}_2 \hat{n} \cdot \vec{S}_1 + \frac{4}{35} (\vec{S}_1 \cdot \vec{v}_1)^2 - \frac{2}{7} (\hat{n} \cdot \vec{v}_1)^2 \vec{S}_1 \cdot \vec{S}_1 + \\
 & \quad \left. \frac{9}{14} \hat{n} \cdot \vec{v}_1 \hat{n} \cdot \vec{v}_2 \vec{S}_1 \cdot \vec{S}_1 - \frac{9}{35} \vec{S}_1 \cdot \vec{v}_1 \vec{S}_1 \cdot \vec{v}_2 + \frac{2}{35} \vec{S}_1 \cdot \vec{S}_1 \vec{v}_1 \cdot \vec{v}_1 - \frac{9}{70} \vec{S}_1 \cdot \vec{S}_1 \vec{v}_1 \cdot \vec{v}_2 \right) \log \left( \frac{r}{R_0} \right) + \\
 & \quad \frac{1}{\epsilon_d} \left( \frac{1}{r^4} \left( \frac{4}{7} \hat{n} \cdot \vec{S}_1 \hat{n} \cdot \vec{S}_1 \hat{n} \cdot \vec{v}_1 - \frac{4}{35} \vec{S}_1 \cdot \vec{S}_1 \hat{n} \cdot \vec{v}_1 - \hat{n} \cdot \vec{S}_1 \hat{n} \cdot \vec{S}_1 \hat{n} \cdot \vec{v}_2 - \frac{4}{35} \hat{n} \cdot \vec{S}_1 \vec{S}_1 \cdot \vec{v}_1 + \right. \right. \\
 & \quad \left. \frac{1}{5} \hat{n} \cdot \vec{S}_1 \vec{S}_1 \cdot \vec{v}_2 + \frac{1}{5} \hat{n} \cdot \vec{v}_2 \vec{S}_1 \cdot \vec{S}_1 - \frac{4}{35} \hat{n} \cdot \vec{S}_1 \vec{S}_1 \cdot \vec{v}_1 + \frac{1}{5} \hat{n} \cdot \vec{S}_1 \vec{S}_1 \cdot \vec{v}_2 \right) + \frac{1}{r^5} \\
 & \quad \left( -\frac{2}{3} (\hat{n} \cdot \vec{v}_1)^2 (\hat{n} \cdot \vec{S}_1)^2 + \frac{3}{2} \hat{n} \cdot \vec{v}_1 \hat{n} \cdot \vec{v}_2 (\hat{n} \cdot \vec{S}_1)^2 + \frac{2}{21} \vec{v}_1 \cdot \vec{v}_1 (\hat{n} \cdot \vec{S}_1)^2 - \frac{3}{14} \vec{v}_1 \cdot \vec{v}_2 (\hat{n} \cdot \vec{S}_1)^2 + \right. \\
 & \quad \frac{8}{21} \hat{n} \cdot \vec{v}_1 \vec{S}_1 \cdot \vec{v}_1 \hat{n} \cdot \vec{S}_1 - \frac{3}{7} \hat{n} \cdot \vec{v}_2 \vec{S}_1 \cdot \vec{v}_1 \hat{n} \cdot \vec{S}_1 - \frac{3}{7} \hat{n} \cdot \vec{v}_1 \vec{S}_1 \cdot \vec{v}_2 \hat{n} \cdot \vec{S}_1 - \frac{4}{105} (\vec{S}_1 \cdot \vec{v}_1)^2 + \frac{2}{21} (\hat{n} \cdot \vec{v}_1)^2 \vec{S}_1 \cdot \vec{S}_1 - \\
 & \quad \left. \frac{3}{14} \hat{n} \cdot \vec{v}_1 \hat{n} \cdot \vec{v}_2 \vec{S}_1 \cdot \vec{S}_1 + \frac{3}{35} \vec{S}_1 \cdot \vec{v}_1 \vec{S}_1 \cdot \vec{v}_2 - \frac{2}{105} \vec{S}_1 \cdot \vec{S}_1 \vec{v}_1 \cdot \vec{v}_1 + \frac{3}{70} \vec{S}_1 \cdot \vec{S}_1 \vec{v}_1 \cdot \vec{v}_2 \right) \left. \right) \Bigg\} c_{ES^2 1} \}
 \end{aligned}$$

{DiagS1CES2[3, 1, 39],

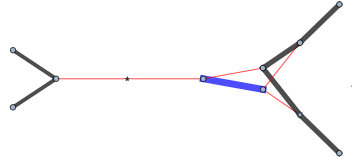

,

$$G^3 m_1 m_2 \left( \frac{\frac{103}{49} \hat{n} \cdot \vec{S}_1 \hat{n} \cdot \vec{S}_1 \hat{n} \cdot \vec{v}_2 - \frac{627 \vec{S}_1 \cdot \vec{S}_1 \hat{n} \cdot \vec{v}_2}{1225} - \frac{452 \hat{n} \cdot \vec{S}_1 \vec{S}_1 \cdot \vec{v}_2}{1225} - \frac{452 \hat{n} \cdot \vec{S}_1 \vec{S}_1 \cdot \vec{v}_2}{1225}}{r^4} + \right.$$

$$\begin{aligned}
& \frac{1}{r^5} \left( -8 \hat{n} \cdot \vec{v}_1 \hat{n} \cdot \vec{v}_2 \left( \hat{n} \cdot \vec{S}_1 \right)^2 + \frac{103}{98} \vec{v}_1 \cdot \vec{v}_2 \left( \hat{n} \cdot \vec{S}_1 \right)^2 + \frac{103}{49} \hat{n} \cdot \vec{v}_2 \vec{S}_1 \cdot \vec{v}_1 \hat{n} \cdot \vec{S}_1 + \right. \\
& \left. \frac{103}{49} \hat{n} \cdot \vec{v}_1 \vec{S}_1 \cdot \vec{v}_2 \hat{n} \cdot \vec{S}_1 + \frac{69}{49} \hat{n} \cdot \vec{v}_1 \hat{n} \cdot \vec{v}_2 \vec{S}_1 \cdot \vec{S}_1 - \frac{452 \vec{S}_1 \cdot \vec{v}_1 \vec{S}_1 \cdot \vec{v}_2}{1225} - \frac{627 \vec{S}_1 \cdot \vec{S}_1 \vec{v}_1 \cdot \vec{v}_2}{2450} \right) + \\
& \left( \frac{-\frac{9}{7} \hat{n} \cdot \vec{S}_1 \hat{n} \cdot \vec{S}_1 \hat{n} \cdot \vec{v}_2 + \frac{9}{35} \vec{S}_1 \cdot \vec{S}_1 \hat{n} \cdot \vec{v}_2 + \frac{9}{35} \hat{n} \cdot \vec{S}_1 \vec{S}_1 \cdot \vec{v}_2 + \frac{9}{35} \hat{n} \cdot \vec{S}_1 \vec{S}_1 \cdot \vec{v}_2}{r^4} + \frac{1}{r^5} \right. \\
& \left( \frac{9}{2} \hat{n} \cdot \vec{v}_1 \hat{n} \cdot \vec{v}_2 \left( \hat{n} \cdot \vec{S}_1 \right)^2 - \frac{9}{14} \vec{v}_1 \cdot \vec{v}_2 \left( \hat{n} \cdot \vec{S}_1 \right)^2 - \frac{9}{7} \hat{n} \cdot \vec{v}_2 \vec{S}_1 \cdot \vec{v}_1 \hat{n} \cdot \vec{S}_1 - \frac{9}{7} \hat{n} \cdot \vec{v}_1 \vec{S}_1 \cdot \vec{v}_2 \hat{n} \cdot \vec{S}_1 - \right. \\
& \left. \frac{9}{14} \hat{n} \cdot \vec{v}_1 \hat{n} \cdot \vec{v}_2 \vec{S}_1 \cdot \vec{S}_1 + \frac{9}{35} \vec{S}_1 \cdot \vec{v}_1 \vec{S}_1 \cdot \vec{v}_2 + \frac{9}{70} \vec{S}_1 \cdot \vec{S}_1 \vec{v}_1 \cdot \vec{v}_2 \right) \log \left( \frac{r}{R_0} \right) + \\
& \frac{1}{\epsilon_d} \left( \frac{\frac{3}{7} \hat{n} \cdot \vec{S}_1 \hat{n} \cdot \vec{S}_1 \hat{n} \cdot \vec{v}_2 - \frac{3}{35} \vec{S}_1 \cdot \vec{S}_1 \hat{n} \cdot \vec{v}_2 - \frac{3}{35} \hat{n} \cdot \vec{S}_1 \vec{S}_1 \cdot \vec{v}_2 - \frac{3}{35} \hat{n} \cdot \vec{S}_1 \vec{S}_1 \cdot \vec{v}_2}{r^4} + \frac{1}{r^5} \right. \\
& \left( -\frac{3}{2} \hat{n} \cdot \vec{v}_1 \hat{n} \cdot \vec{v}_2 \left( \hat{n} \cdot \vec{S}_1 \right)^2 + \frac{3}{14} \vec{v}_1 \cdot \vec{v}_2 \left( \hat{n} \cdot \vec{S}_1 \right)^2 + \frac{3}{7} \hat{n} \cdot \vec{v}_2 \vec{S}_1 \cdot \vec{v}_1 \hat{n} \cdot \vec{S}_1 + \right. \\
& \left. \left. \frac{3}{7} \hat{n} \cdot \vec{v}_1 \vec{S}_1 \cdot \vec{v}_2 \hat{n} \cdot \vec{S}_1 + \frac{3}{14} \hat{n} \cdot \vec{v}_1 \hat{n} \cdot \vec{v}_2 \vec{S}_1 \cdot \vec{S}_1 - \frac{3}{35} \vec{S}_1 \cdot \vec{v}_1 \vec{S}_1 \cdot \vec{v}_2 - \frac{3}{70} \vec{S}_1 \cdot \vec{S}_1 \vec{v}_1 \cdot \vec{v}_2 \right) \right) \Bigg\} c_{\text{ES}^2 1} \}
\end{aligned}$$

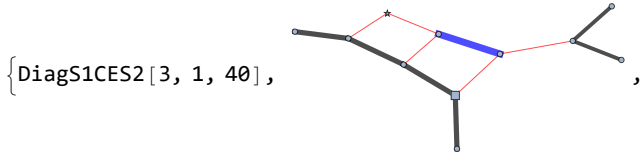

$$\begin{aligned}
& G^3 m_1 m_2 \left( \frac{-\frac{1961}{147} \hat{n} \cdot \vec{S}_1 \hat{n} \cdot \vec{S}_1 \hat{n} \cdot \vec{v}_1 + \frac{12262 \vec{S}_1 \cdot \vec{S}_1 \hat{n} \cdot \vec{v}_1}{3675} + \frac{18749 \hat{n} \cdot \vec{S}_1 \vec{S}_1 \cdot \vec{v}_1}{7350} + \frac{18749 \hat{n} \cdot \vec{S}_1 \vec{S}_1 \cdot \vec{v}_1}{7350}}{r^4} + \frac{1}{r^5} \right. \\
& \left( \frac{113}{2} \left( \hat{n} \cdot \vec{v}_1 \right)^2 \left( \hat{n} \cdot \vec{S}_1 \right)^2 - \frac{160}{3} \hat{n} \cdot \vec{v}_1 \hat{n} \cdot \vec{v}_2 \left( \hat{n} \cdot \vec{S}_1 \right)^2 - \frac{2341}{294} \vec{v}_1 \cdot \vec{v}_1 \left( \hat{n} \cdot \vec{S}_1 \right)^2 + \frac{1961}{294} \vec{v}_1 \cdot \vec{v}_2 \left( \hat{n} \cdot \vec{S}_1 \right)^2 - \right. \\
& \frac{8923}{294} \hat{n} \cdot \vec{v}_1 \vec{S}_1 \cdot \vec{v}_1 \hat{n} \cdot \vec{S}_1 + \frac{4531}{294} \hat{n} \cdot \vec{v}_2 \vec{S}_1 \cdot \vec{v}_1 \hat{n} \cdot \vec{S}_1 + \frac{1961}{147} \hat{n} \cdot \vec{v}_1 \vec{S}_1 \cdot \vec{v}_2 \hat{n} \cdot \vec{S}_1 + \frac{3302 \left( \vec{S}_1 \cdot \vec{v}_1 \right)^2}{1225} - \frac{508}{49} \left( \hat{n} \cdot \vec{v}_1 \right)^2 \\
& \left. \vec{S}_1 \cdot \vec{S}_1 + \frac{2843}{294} \hat{n} \cdot \vec{v}_1 \hat{n} \cdot \vec{v}_2 \vec{S}_1 \cdot \vec{S}_1 - \frac{18749 \vec{S}_1 \cdot \vec{v}_1 \vec{S}_1 \cdot \vec{v}_2}{7350} + \frac{15331 \vec{S}_1 \cdot \vec{S}_1 \vec{v}_1 \cdot \vec{v}_1}{7350} - \frac{6131 \vec{S}_1 \cdot \vec{S}_1 \vec{v}_1 \cdot \vec{v}_2}{3675} \right) + \\
& \left( \frac{\frac{93}{7} \hat{n} \cdot \vec{S}_1 \hat{n} \cdot \vec{S}_1 \hat{n} \cdot \vec{v}_1 - \frac{93}{35} \vec{S}_1 \cdot \vec{S}_1 \hat{n} \cdot \vec{v}_1 - \frac{93}{35} \hat{n} \cdot \vec{S}_1 \vec{S}_1 \cdot \vec{v}_1 - \frac{93}{35} \hat{n} \cdot \vec{S}_1 \vec{S}_1 \cdot \vec{v}_1}{r^4} + \frac{1}{r^5} \right. \\
& \left( -52 \left( \hat{n} \cdot \vec{v}_1 \right)^2 \left( \hat{n} \cdot \vec{S}_1 \right)^2 + \frac{93}{2} \hat{n} \cdot \vec{v}_1 \hat{n} \cdot \vec{v}_2 \left( \hat{n} \cdot \vec{S}_1 \right)^2 + \frac{52}{7} \vec{v}_1 \cdot \vec{v}_1 \left( \hat{n} \cdot \vec{S}_1 \right)^2 - \frac{93}{14} \vec{v}_1 \cdot \vec{v}_2 \left( \hat{n} \cdot \vec{S}_1 \right)^2 + \right. \\
& \left. \frac{208}{7} \hat{n} \cdot \vec{v}_1 \vec{S}_1 \cdot \vec{v}_1 \hat{n} \cdot \vec{S}_1 - \frac{93}{7} \hat{n} \cdot \vec{v}_2 \vec{S}_1 \cdot \vec{v}_1 \hat{n} \cdot \vec{S}_1 - \frac{93}{7} \hat{n} \cdot \vec{v}_1 \vec{S}_1 \cdot \vec{v}_2 \hat{n} \cdot \vec{S}_1 - \frac{104}{35} \left( \vec{S}_1 \cdot \vec{v}_1 \right)^2 + \right.
\end{aligned}$$

$$\left. \begin{aligned} & \frac{52}{7} (\hat{n} \cdot \vec{v}_1)^2 \vec{S}_1 \cdot \vec{S}_1 - \frac{93}{14} \hat{n} \cdot \vec{v}_1 \hat{n} \cdot \vec{v}_2 \vec{S}_1 \cdot \vec{S}_1 + \frac{93}{35} \vec{S}_1 \cdot \vec{v}_1 \vec{S}_1 \cdot \vec{v}_2 - \frac{52}{35} \vec{S}_1 \cdot \vec{S}_1 \vec{v}_1 \cdot \vec{v}_1 + \frac{93}{70} \vec{S}_1 \cdot \vec{S}_1 \vec{v}_1 \cdot \vec{v}_2 \Bigg) \\ & \log \left( \frac{r}{R_0} \right) + \frac{1}{\epsilon_d} \left( \frac{-\frac{31}{7} \hat{n} \cdot \vec{S}_1 \hat{n} \cdot \vec{S}_1 \hat{n} \cdot \vec{v}_1 + \frac{31}{35} \vec{S}_1 \cdot \vec{S}_1 \hat{n} \cdot \vec{v}_1 + \frac{31}{35} \hat{n} \cdot \vec{S}_1 \vec{S}_1 \cdot \vec{v}_1 + \frac{31}{35} \hat{n} \cdot \vec{S}_1 \vec{S}_1 \cdot \vec{v}_1}{r^4} + \frac{1}{r^5} \right. \\ & \left( \frac{52}{3} (\hat{n} \cdot \vec{v}_1)^2 (\hat{n} \cdot \vec{S}_1)^2 - \frac{31}{2} \hat{n} \cdot \vec{v}_1 \hat{n} \cdot \vec{v}_2 (\hat{n} \cdot \vec{S}_1)^2 - \frac{52}{21} \vec{v}_1 \cdot \vec{v}_1 (\hat{n} \cdot \vec{S}_1)^2 + \frac{31}{14} \vec{v}_1 \cdot \vec{v}_2 (\hat{n} \cdot \vec{S}_1)^2 - \right. \\ & \frac{208}{21} \hat{n} \cdot \vec{v}_1 \vec{S}_1 \cdot \vec{v}_1 \hat{n} \cdot \vec{S}_1 + \frac{31}{7} \hat{n} \cdot \vec{v}_2 \vec{S}_1 \cdot \vec{v}_1 \hat{n} \cdot \vec{S}_1 + \frac{31}{7} \hat{n} \cdot \vec{v}_1 \vec{S}_1 \cdot \vec{v}_2 \hat{n} \cdot \vec{S}_1 + \frac{104}{105} (\vec{S}_1 \cdot \vec{v}_1)^2 - \frac{52}{21} (\hat{n} \cdot \vec{v}_1)^2 \\ & \left. \left. \left. \vec{S}_1 \cdot \vec{S}_1 + \frac{31}{14} \hat{n} \cdot \vec{v}_1 \hat{n} \cdot \vec{v}_2 \vec{S}_1 \cdot \vec{S}_1 - \frac{31}{35} \vec{S}_1 \cdot \vec{v}_1 \vec{S}_1 \cdot \vec{v}_2 + \frac{52}{105} \vec{S}_1 \cdot \vec{S}_1 \vec{v}_1 \cdot \vec{v}_1 - \frac{31}{70} \vec{S}_1 \cdot \vec{S}_1 \vec{v}_1 \cdot \vec{v}_2 \right) \right) \right) \Bigg\} c_{\text{ES}^2 1} \end{aligned} \right)$$

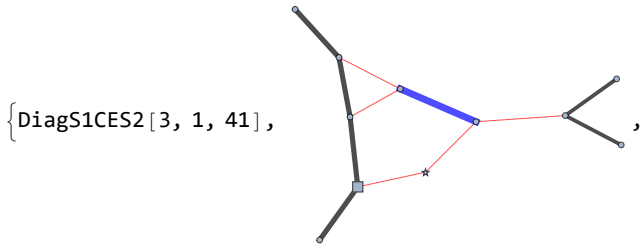

$$\begin{aligned} & G^3 m_1 m_2 \left( \frac{1}{r^4} \left( -\frac{15}{98} \hat{n} \cdot \vec{S}_1 \hat{n} \cdot \vec{S}_1 \hat{n} \cdot \vec{v}_1 + \frac{523 \vec{S}_1 \cdot \vec{S}_1 \hat{n} \cdot \vec{v}_1}{2450} - \frac{15}{4} \hat{n} \cdot \vec{S}_1 \hat{n} \cdot \vec{S}_1 \hat{n} \cdot \vec{v}_2 + \right. \right. \\ & \left. \frac{453 \hat{n} \cdot \vec{S}_1 \vec{S}_1 \cdot \vec{v}_1}{2450} + \frac{69}{100} \hat{n} \cdot \vec{S}_1 \vec{S}_1 \cdot \vec{v}_2 + \frac{19}{100} \hat{n} \cdot \vec{v}_2 \vec{S}_1 \cdot \vec{S}_1 + \frac{453 \hat{n} \cdot \vec{S}_1 \vec{S}_1 \cdot \vec{v}_1}{2450} + \frac{69}{100} \hat{n} \cdot \vec{S}_1 \vec{S}_1 \cdot \vec{v}_2 \right) + \frac{1}{r^5} \\ & \left( \frac{1}{24} (\hat{n} \cdot \vec{v}_1)^2 (\hat{n} \cdot \vec{S}_1)^2 + \frac{117}{8} \hat{n} \cdot \vec{v}_1 \hat{n} \cdot \vec{v}_2 (\hat{n} \cdot \vec{S}_1)^2 - \frac{325 \vec{v}_1 \cdot \vec{v}_1 (\hat{n} \cdot \vec{S}_1)^2}{1176} - \frac{765}{392} \vec{v}_1 \cdot \vec{v}_2 (\hat{n} \cdot \vec{S}_1)^2 - \right. \\ & \frac{73}{294} \hat{n} \cdot \vec{v}_1 \vec{S}_1 \cdot \vec{v}_1 \hat{n} \cdot \vec{S}_1 - \frac{933}{196} \hat{n} \cdot \vec{v}_2 \vec{S}_1 \cdot \vec{v}_1 \hat{n} \cdot \vec{S}_1 - \frac{765}{196} \hat{n} \cdot \vec{v}_1 \vec{S}_1 \cdot \vec{v}_2 \hat{n} \cdot \vec{S}_1 + \frac{2339 (\vec{S}_1 \cdot \vec{v}_1)^2}{14700} - \\ & \left. \frac{115 (\hat{n} \cdot \vec{v}_1)^2 \vec{S}_1 \cdot \vec{S}_1}{1176} - \frac{471}{392} \hat{n} \cdot \vec{v}_1 \hat{n} \cdot \vec{v}_2 \vec{S}_1 \cdot \vec{S}_1 + \frac{4287 \vec{S}_1 \cdot \vec{v}_1 \vec{S}_1 \cdot \vec{v}_2}{4900} - \frac{1231 \vec{S}_1 \cdot \vec{S}_1 \vec{v}_1 \cdot \vec{v}_1}{29400} + \frac{1977 \vec{S}_1 \cdot \vec{S}_1 \vec{v}_1 \cdot \vec{v}_2}{9800} \right) + \\ & \left( \frac{1}{r^4} \left( \frac{3}{7} \hat{n} \cdot \vec{S}_1 \hat{n} \cdot \vec{S}_1 \hat{n} \cdot \vec{v}_1 - \frac{3}{35} \vec{S}_1 \cdot \vec{S}_1 \hat{n} \cdot \vec{v}_1 + \frac{3}{2} \hat{n} \cdot \vec{S}_1 \hat{n} \cdot \vec{S}_1 \hat{n} \cdot \vec{v}_2 - \frac{3}{35} \hat{n} \cdot \vec{S}_1 \vec{S}_1 \cdot \vec{v}_1 - \right. \right. \\ & \left. \frac{3}{10} \hat{n} \cdot \vec{S}_1 \vec{S}_1 \cdot \vec{v}_2 - \frac{3}{10} \hat{n} \cdot \vec{v}_2 \vec{S}_1 \cdot \vec{S}_1 - \frac{3}{35} \hat{n} \cdot \vec{S}_1 \vec{S}_1 \cdot \vec{v}_1 - \frac{3}{10} \hat{n} \cdot \vec{S}_1 \vec{S}_1 \cdot \vec{v}_2 \right) + \frac{1}{r^5} \\ & \left( -\frac{3}{4} (\hat{n} \cdot \vec{v}_1)^2 (\hat{n} \cdot \vec{S}_1)^2 - \frac{27}{4} \hat{n} \cdot \vec{v}_1 \hat{n} \cdot \vec{v}_2 (\hat{n} \cdot \vec{S}_1)^2 + \frac{3}{28} \vec{v}_1 \cdot \vec{v}_1 (\hat{n} \cdot \vec{S}_1)^2 + \frac{27}{28} \vec{v}_1 \cdot \vec{v}_2 (\hat{n} \cdot \vec{S}_1)^2 + \right. \\ & \frac{3}{7} \hat{n} \cdot \vec{v}_1 \vec{S}_1 \cdot \vec{v}_1 \hat{n} \cdot \vec{S}_1 + \frac{27}{14} \hat{n} \cdot \vec{v}_2 \vec{S}_1 \cdot \vec{v}_1 \hat{n} \cdot \vec{S}_1 + \frac{27}{14} \hat{n} \cdot \vec{v}_1 \vec{S}_1 \cdot \vec{v}_2 \hat{n} \cdot \vec{S}_1 - \frac{3}{70} (\vec{S}_1 \cdot \vec{v}_1)^2 + \frac{3}{28} (\hat{n} \cdot \vec{v}_1)^2 \vec{S}_1 \cdot \vec{S}_1 + \\ & \left. \frac{27}{28} \hat{n} \cdot \vec{v}_1 \hat{n} \cdot \vec{v}_2 \vec{S}_1 \cdot \vec{S}_1 - \frac{27}{70} \vec{S}_1 \cdot \vec{v}_1 \vec{S}_1 \cdot \vec{v}_2 - \frac{3}{140} \vec{S}_1 \cdot \vec{S}_1 \vec{v}_1 \cdot \vec{v}_1 - \frac{27}{140} \vec{S}_1 \cdot \vec{S}_1 \vec{v}_1 \cdot \vec{v}_2 \right) \log \left( \frac{r}{R_0} \right) + \\ & \frac{1}{\epsilon_d} \left( \frac{1}{r^4} \left( -\frac{1}{7} \hat{n} \cdot \vec{S}_1 \hat{n} \cdot \vec{S}_1 \hat{n} \cdot \vec{v}_1 + \frac{1}{35} \vec{S}_1 \cdot \vec{S}_1 \hat{n} \cdot \vec{v}_1 - \frac{1}{2} \hat{n} \cdot \vec{S}_1 \hat{n} \cdot \vec{S}_1 \hat{n} \cdot \vec{v}_2 + \frac{1}{35} \hat{n} \cdot \vec{S}_1 \vec{S}_1 \cdot \vec{v}_1 + \right. \right. \end{aligned}$$

$$\begin{aligned} & \left. \left( \frac{1}{10} \hat{n} \cdot \vec{S}_1 \vec{S}_1 \cdot \vec{v}_2 + \frac{1}{10} \hat{n} \cdot \vec{v}_2 \vec{S}_1 \cdot \vec{S}_1 + \frac{1}{35} \hat{n} \cdot \vec{S}_1 \vec{S}_1 \cdot \vec{v}_1 + \frac{1}{10} \hat{n} \cdot \vec{S}_1 \vec{S}_1 \cdot \vec{v}_2 \right) + \frac{1}{r^5} \right. \\ & \left( \frac{1}{4} (\hat{n} \cdot \vec{v}_1)^2 (\hat{n} \cdot \vec{S}_1)^2 + \frac{9}{4} \hat{n} \cdot \vec{v}_1 \hat{n} \cdot \vec{v}_2 (\hat{n} \cdot \vec{S}_1)^2 - \frac{1}{28} \vec{v}_1 \cdot \vec{v}_1 (\hat{n} \cdot \vec{S}_1)^2 - \frac{9}{28} \vec{v}_1 \cdot \vec{v}_2 (\hat{n} \cdot \vec{S}_1)^2 - \right. \\ & \frac{1}{7} \hat{n} \cdot \vec{v}_1 \vec{S}_1 \cdot \vec{v}_1 \hat{n} \cdot \vec{S}_1 - \frac{9}{14} \hat{n} \cdot \vec{v}_2 \vec{S}_1 \cdot \vec{v}_1 \hat{n} \cdot \vec{S}_1 - \frac{9}{14} \hat{n} \cdot \vec{v}_1 \vec{S}_1 \cdot \vec{v}_2 \hat{n} \cdot \vec{S}_1 + \frac{1}{70} (\vec{S}_1 \cdot \vec{v}_1)^2 - \frac{1}{28} (\hat{n} \cdot \vec{v}_1)^2 \vec{S}_1 \cdot \vec{S}_1 - \\ & \left. \left. \frac{9}{28} \hat{n} \cdot \vec{v}_1 \hat{n} \cdot \vec{v}_2 \vec{S}_1 \cdot \vec{S}_1 + \frac{9}{70} \vec{S}_1 \cdot \vec{v}_1 \vec{S}_1 \cdot \vec{v}_2 + \frac{1}{140} \vec{S}_1 \cdot \vec{S}_1 \vec{v}_1 \cdot \vec{v}_1 + \frac{9}{140} \vec{S}_1 \cdot \vec{S}_1 \vec{v}_1 \cdot \vec{v}_2 \right) \right) \Bigg) \Bigg\} c_{\text{ES}^2 1} \end{aligned}$$

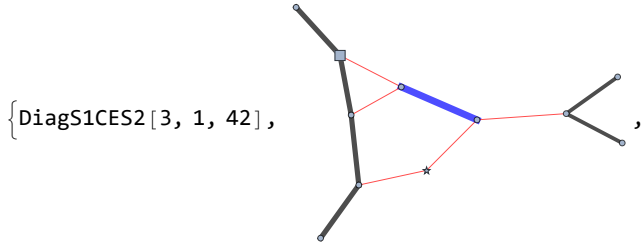

$$\begin{aligned} & G^3 m_1 m_2 \left( \frac{-\frac{43}{49} \hat{n} \cdot \vec{S}_1 \hat{n} \cdot \vec{S}_1 \hat{n} \cdot \vec{v}_1 + \frac{173 \vec{S}_1 \cdot \vec{S}_1 \hat{n} \cdot \vec{v}_1}{1225} + \frac{348 \hat{n} \cdot \vec{S}_1 \vec{S}_1 \cdot \vec{v}_1}{1225} + \frac{348 \hat{n} \cdot \vec{S}_1 \vec{S}_1 \cdot \vec{v}_1}{1225}}{r^4} + \frac{1}{r^5} \right. \\ & \left( \frac{131}{48} (\hat{n} \cdot \vec{v}_1)^2 (\hat{n} \cdot \vec{S}_1)^2 - \frac{7}{2} \hat{n} \cdot \vec{v}_1 \hat{n} \cdot \vec{v}_2 (\hat{n} \cdot \vec{S}_1)^2 - \frac{1313 \vec{v}_1 \cdot \vec{v}_1 (\hat{n} \cdot \vec{S}_1)^2}{2352} + \frac{43}{98} \vec{v}_1 \cdot \vec{v}_2 (\hat{n} \cdot \vec{S}_1)^2 - \right. \\ & \frac{1061}{588} \hat{n} \cdot \vec{v}_1 \vec{S}_1 \cdot \vec{v}_1 \hat{n} \cdot \vec{S}_1 + \frac{78}{49} \hat{n} \cdot \vec{v}_2 \vec{S}_1 \cdot \vec{v}_1 \hat{n} \cdot \vec{S}_1 + \frac{43}{49} \hat{n} \cdot \vec{v}_1 \vec{S}_1 \cdot \vec{v}_2 \hat{n} \cdot \vec{S}_1 + \frac{8329 (\vec{S}_1 \cdot \vec{v}_1)^2}{29400} - \\ & \left. \frac{893 (\hat{n} \cdot \vec{v}_1)^2 \vec{S}_1 \cdot \vec{S}_1}{2352} + \frac{43}{98} \hat{n} \cdot \vec{v}_1 \hat{n} \cdot \vec{v}_2 \vec{S}_1 \cdot \vec{S}_1 - \frac{348 \vec{S}_1 \cdot \vec{v}_1 \vec{S}_1 \cdot \vec{v}_2}{1225} + \frac{6229 \vec{S}_1 \cdot \vec{S}_1 \vec{v}_1 \cdot \vec{v}_1}{58800} - \frac{173 \vec{S}_1 \cdot \vec{S}_1 \vec{v}_1 \cdot \vec{v}_2}{2450} \right) + \\ & \left( \frac{\frac{6}{7} \hat{n} \cdot \vec{S}_1 \hat{n} \cdot \vec{S}_1 \hat{n} \cdot \vec{v}_1 - \frac{6}{35} \vec{S}_1 \cdot \vec{S}_1 \hat{n} \cdot \vec{v}_1 - \frac{6}{35} \hat{n} \cdot \vec{S}_1 \vec{S}_1 \cdot \vec{v}_1 - \frac{6}{35} \hat{n} \cdot \vec{S}_1 \vec{S}_1 \cdot \vec{v}_1}{r^4} + \frac{1}{r^5} \right. \\ & \left( -\frac{9}{4} (\hat{n} \cdot \vec{v}_1)^2 (\hat{n} \cdot \vec{S}_1)^2 + 3 \hat{n} \cdot \vec{v}_1 \hat{n} \cdot \vec{v}_2 (\hat{n} \cdot \vec{S}_1)^2 + \frac{9}{28} \vec{v}_1 \cdot \vec{v}_1 (\hat{n} \cdot \vec{S}_1)^2 - \frac{3}{7} \vec{v}_1 \cdot \vec{v}_2 (\hat{n} \cdot \vec{S}_1)^2 + \right. \\ & \frac{9}{7} \hat{n} \cdot \vec{v}_1 \vec{S}_1 \cdot \vec{v}_1 \hat{n} \cdot \vec{S}_1 - \frac{6}{7} \hat{n} \cdot \vec{v}_2 \vec{S}_1 \cdot \vec{v}_1 \hat{n} \cdot \vec{S}_1 - \frac{6}{7} \hat{n} \cdot \vec{v}_1 \vec{S}_1 \cdot \vec{v}_2 \hat{n} \cdot \vec{S}_1 - \frac{9}{70} (\vec{S}_1 \cdot \vec{v}_1)^2 + \frac{9}{28} (\hat{n} \cdot \vec{v}_1)^2 \vec{S}_1 \cdot \vec{S}_1 - \\ & \left. \frac{3}{7} \hat{n} \cdot \vec{v}_1 \hat{n} \cdot \vec{v}_2 \vec{S}_1 \cdot \vec{S}_1 + \frac{6}{35} \vec{S}_1 \cdot \vec{v}_1 \vec{S}_1 \cdot \vec{v}_2 - \frac{9}{140} \vec{S}_1 \cdot \vec{S}_1 \vec{v}_1 \cdot \vec{v}_1 + \frac{3}{35} \vec{S}_1 \cdot \vec{S}_1 \vec{v}_1 \cdot \vec{v}_2 \right) \log \left( \frac{r}{R_\theta} \right) + \\ & \frac{1}{\epsilon_d} \left( \frac{-\frac{2}{7} \hat{n} \cdot \vec{S}_1 \hat{n} \cdot \vec{S}_1 \hat{n} \cdot \vec{v}_1 + \frac{2}{35} \vec{S}_1 \cdot \vec{S}_1 \hat{n} \cdot \vec{v}_1 + \frac{2}{35} \hat{n} \cdot \vec{S}_1 \vec{S}_1 \cdot \vec{v}_1 + \frac{2}{35} \hat{n} \cdot \vec{S}_1 \vec{S}_1 \cdot \vec{v}_1}{r^4} + \frac{1}{r^5} \right. \\ & \left( \frac{3}{4} (\hat{n} \cdot \vec{v}_1)^2 (\hat{n} \cdot \vec{S}_1)^2 - \hat{n} \cdot \vec{v}_1 \hat{n} \cdot \vec{v}_2 (\hat{n} \cdot \vec{S}_1)^2 - \frac{3}{28} \vec{v}_1 \cdot \vec{v}_1 (\hat{n} \cdot \vec{S}_1)^2 + \frac{1}{7} \vec{v}_1 \cdot \vec{v}_2 (\hat{n} \cdot \vec{S}_1)^2 - \right. \\ & \left. \frac{3}{7} \hat{n} \cdot \vec{v}_1 \vec{S}_1 \cdot \vec{v}_1 \hat{n} \cdot \vec{S}_1 + \frac{2}{7} \hat{n} \cdot \vec{v}_2 \vec{S}_1 \cdot \vec{v}_1 \hat{n} \cdot \vec{S}_1 + \frac{2}{7} \hat{n} \cdot \vec{v}_1 \vec{S}_1 \cdot \vec{v}_2 \hat{n} \cdot \vec{S}_1 + \frac{3}{70} (\vec{S}_1 \cdot \vec{v}_1)^2 - \frac{3}{28} (\hat{n} \cdot \vec{v}_1)^2 \vec{S}_1 \cdot \vec{S}_1 + \right. \end{aligned}$$

$$\left. \left. \left. \frac{1}{7} \hat{n} \cdot \vec{v}_1 \hat{n} \cdot \vec{v}_2 \vec{S}_1 \cdot \vec{S}_1 - \frac{2}{35} \vec{S}_1 \cdot \vec{v}_1 \vec{S}_1 \cdot \vec{v}_2 + \frac{3}{140} \vec{S}_1 \cdot \vec{S}_1 \vec{v}_1 \cdot \vec{v}_1 - \frac{1}{35} \vec{S}_1 \cdot \vec{S}_1 \vec{v}_1 \cdot \vec{v}_2 \right) \right) \right\} c_{ES^2 1} \}$$

{DiagS1CES2[3, 1, 43],

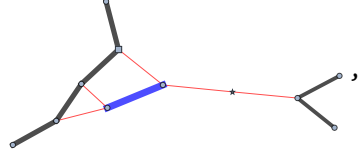

$$G^3 m_1 m_2 \left( \frac{\frac{1005}{196} \hat{n} \cdot \vec{S}_1 \hat{n} \cdot \vec{S}_1 \hat{n} \cdot \vec{v}_2 - \frac{6369}{4900} \vec{S}_1 \cdot \vec{S}_1 \hat{n} \cdot \vec{v}_2 - \frac{4269}{4900} \hat{n} \cdot \vec{S}_1 \vec{S}_1 \cdot \vec{v}_2 - \frac{4269}{4900} \hat{n} \cdot \vec{S}_1 \vec{S}_1 \cdot \vec{v}_2}{r^4} + \right.$$

$$\frac{1}{r^5} \left( -\frac{159}{8} \hat{n} \cdot \vec{v}_1 \hat{n} \cdot \vec{v}_2 (\hat{n} \cdot \vec{S}_1)^2 + \frac{1005}{392} \vec{v}_1 \cdot \vec{v}_2 (\hat{n} \cdot \vec{S}_1)^2 + \frac{1005}{196} \hat{n} \cdot \vec{v}_2 \vec{S}_1 \cdot \vec{v}_1 \hat{n} \cdot \vec{S}_1 + \right.$$

$$\frac{1005}{196} \hat{n} \cdot \vec{v}_1 \vec{S}_1 \cdot \vec{v}_2 \hat{n} \cdot \vec{S}_1 + \frac{1425}{392} \hat{n} \cdot \vec{v}_1 \hat{n} \cdot \vec{v}_2 \vec{S}_1 \cdot \vec{S}_1 - \frac{4269}{4900} \vec{S}_1 \cdot \vec{v}_1 \vec{S}_1 \cdot \vec{v}_2 - \frac{6369}{9800} \vec{S}_1 \cdot \vec{S}_1 \vec{v}_1 \cdot \vec{v}_2 \Big) +$$

$$\left( \frac{-\frac{27}{7} \hat{n} \cdot \vec{S}_1 \hat{n} \cdot \vec{S}_1 \hat{n} \cdot \vec{v}_2 + \frac{27}{35} \vec{S}_1 \cdot \vec{S}_1 \hat{n} \cdot \vec{v}_2 + \frac{27}{35} \hat{n} \cdot \vec{S}_1 \vec{S}_1 \cdot \vec{v}_2 + \frac{27}{35} \hat{n} \cdot \vec{S}_1 \vec{S}_1 \cdot \vec{v}_2}{r^4} + \frac{1}{r^5} \right.$$

$$\left( \frac{27}{2} \hat{n} \cdot \vec{v}_1 \hat{n} \cdot \vec{v}_2 (\hat{n} \cdot \vec{S}_1)^2 - \frac{27}{14} \vec{v}_1 \cdot \vec{v}_2 (\hat{n} \cdot \vec{S}_1)^2 - \frac{27}{7} \hat{n} \cdot \vec{v}_2 \vec{S}_1 \cdot \vec{v}_1 \hat{n} \cdot \vec{S}_1 - \frac{27}{7} \hat{n} \cdot \vec{v}_1 \vec{S}_1 \cdot \vec{v}_2 \hat{n} \cdot \vec{S}_1 - \right.$$

$$\left. \frac{27}{14} \hat{n} \cdot \vec{v}_1 \hat{n} \cdot \vec{v}_2 \vec{S}_1 \cdot \vec{S}_1 + \frac{27}{35} \vec{S}_1 \cdot \vec{v}_1 \vec{S}_1 \cdot \vec{v}_2 + \frac{27}{70} \vec{S}_1 \cdot \vec{S}_1 \vec{v}_1 \cdot \vec{v}_2 \right) \log \left( \frac{r}{R_\theta} \right) +$$

$$\frac{1}{\epsilon_d} \left( \frac{\frac{9}{7} \hat{n} \cdot \vec{S}_1 \hat{n} \cdot \vec{S}_1 \hat{n} \cdot \vec{v}_2 - \frac{9}{35} \vec{S}_1 \cdot \vec{S}_1 \hat{n} \cdot \vec{v}_2 - \frac{9}{35} \hat{n} \cdot \vec{S}_1 \vec{S}_1 \cdot \vec{v}_2 - \frac{9}{35} \hat{n} \cdot \vec{S}_1 \vec{S}_1 \cdot \vec{v}_2}{r^4} + \frac{1}{r^5} \right.$$

$$\left( -\frac{9}{2} \hat{n} \cdot \vec{v}_1 \hat{n} \cdot \vec{v}_2 (\hat{n} \cdot \vec{S}_1)^2 + \frac{9}{14} \vec{v}_1 \cdot \vec{v}_2 (\hat{n} \cdot \vec{S}_1)^2 + \frac{9}{7} \hat{n} \cdot \vec{v}_2 \vec{S}_1 \cdot \vec{v}_1 \hat{n} \cdot \vec{S}_1 + \right.$$

$$\left. \frac{9}{7} \hat{n} \cdot \vec{v}_1 \vec{S}_1 \cdot \vec{v}_2 \hat{n} \cdot \vec{S}_1 + \frac{9}{14} \hat{n} \cdot \vec{v}_1 \hat{n} \cdot \vec{v}_2 \vec{S}_1 \cdot \vec{S}_1 - \frac{9}{35} \vec{S}_1 \cdot \vec{v}_1 \vec{S}_1 \cdot \vec{v}_2 - \frac{9}{70} \vec{S}_1 \cdot \vec{S}_1 \vec{v}_1 \cdot \vec{v}_2 \right) \Big) \Big) c_{ES^2 1} \}$$

{DiagS1CES2[3, 1, 44],

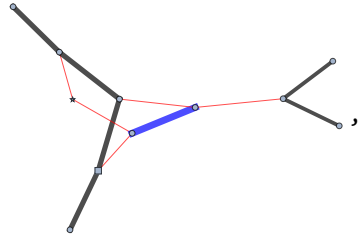

$$G^3 m_1 m_2 \left( \frac{-\frac{775}{294} \hat{n} \cdot \vec{S}_1 \hat{n} \cdot \vec{S}_1 \hat{n} \cdot \vec{v}_1 + \frac{4841}{7350} \vec{S}_1 \cdot \vec{S}_1 \hat{n} \cdot \vec{v}_1 + \frac{1633}{3675} \hat{n} \cdot \vec{S}_1 \vec{S}_1 \cdot \vec{v}_1 + \frac{1633}{3675} \hat{n} \cdot \vec{S}_1 \vec{S}_1 \cdot \vec{v}_1}{r^4} + \frac{1}{r^5} \right.$$

$$\left( \frac{413}{48} (\hat{n} \cdot \vec{v}_1)^2 (\hat{n} \cdot \vec{S}_1)^2 - \frac{121}{12} \hat{n} \cdot \vec{v}_1 \hat{n} \cdot \vec{v}_2 (\hat{n} \cdot \vec{S}_1)^2 - \frac{71}{48} \vec{v}_1 \cdot \vec{v}_1 (\hat{n} \cdot \vec{S}_1)^2 + \frac{775}{588} \vec{v}_1 \cdot \vec{v}_2 (\hat{n} \cdot \vec{S}_1)^2 - \right.$$

$$\begin{aligned}
& \frac{311}{84} \hat{n} \cdot \vec{v}_1 \vec{S}_1 \cdot \vec{v}_1 \hat{n} \cdot \vec{S}_1 + \frac{377}{147} \hat{n} \cdot \vec{v}_2 \vec{S}_1 \cdot \vec{v}_1 \hat{n} \cdot \vec{S}_1 + \frac{775}{294} \hat{n} \cdot \vec{v}_1 \vec{S}_1 \cdot \vec{v}_2 \hat{n} \cdot \vec{S}_1 + \frac{673}{4200} (\vec{S}_1 \cdot \vec{v}_1)^2 - \frac{605}{336} (\hat{n} \cdot \vec{v}_1)^2 \\
& \left. \vec{S}_1 \cdot \vec{S}_1 + \frac{1069}{588} \hat{n} \cdot \vec{v}_1 \hat{n} \cdot \vec{v}_2 \vec{S}_1 \cdot \vec{S}_1 - \frac{1633 \vec{S}_1 \cdot \vec{v}_1 \vec{S}_1 \cdot \vec{v}_2}{3675} + \frac{3973 \vec{S}_1 \cdot \vec{S}_1 \vec{v}_1 \cdot \vec{v}_1}{8400} - \frac{4841 \vec{S}_1 \cdot \vec{S}_1 \vec{v}_1 \cdot \vec{v}_2}{14700} \right) + \\
& \left( \frac{\frac{12}{7} \hat{n} \cdot \vec{S}_1 \hat{n} \cdot \vec{S}_1 \hat{n} \cdot \vec{v}_1 - \frac{12}{35} \vec{S}_1 \cdot \vec{S}_1 \hat{n} \cdot \vec{v}_1 - \frac{12}{35} \hat{n} \cdot \vec{S}_1 \vec{S}_1 \cdot \vec{v}_1 - \frac{12}{35} \hat{n} \cdot \vec{S}_1 \vec{S}_1 \cdot \vec{v}_1}{r^4} + \frac{1}{r^5} \right. \\
& \left( -\frac{21}{4} (\hat{n} \cdot \vec{v}_1)^2 (\hat{n} \cdot \vec{S}_1)^2 + 6 \hat{n} \cdot \vec{v}_1 \hat{n} \cdot \vec{v}_2 (\hat{n} \cdot \vec{S}_1)^2 + \frac{3}{4} \vec{v}_1 \cdot \vec{v}_1 (\hat{n} \cdot \vec{S}_1)^2 - \frac{6}{7} \vec{v}_1 \cdot \vec{v}_2 (\hat{n} \cdot \vec{S}_1)^2 + \right. \\
& 3 \hat{n} \cdot \vec{v}_1 \vec{S}_1 \cdot \vec{v}_1 \hat{n} \cdot \vec{S}_1 - \frac{12}{7} \hat{n} \cdot \vec{v}_2 \vec{S}_1 \cdot \vec{v}_1 \hat{n} \cdot \vec{S}_1 - \frac{12}{7} \hat{n} \cdot \vec{v}_1 \vec{S}_1 \cdot \vec{v}_2 \hat{n} \cdot \vec{S}_1 - \frac{3}{10} (\vec{S}_1 \cdot \vec{v}_1)^2 + \frac{3}{4} (\hat{n} \cdot \vec{v}_1)^2 \vec{S}_1 \cdot \vec{S}_1 - \\
& \left. \frac{6}{7} \hat{n} \cdot \vec{v}_1 \hat{n} \cdot \vec{v}_2 \vec{S}_1 \cdot \vec{S}_1 + \frac{12}{35} \vec{S}_1 \cdot \vec{v}_1 \vec{S}_1 \cdot \vec{v}_2 - \frac{3}{20} \vec{S}_1 \cdot \vec{S}_1 \vec{v}_1 \cdot \vec{v}_1 + \frac{6}{35} \vec{S}_1 \cdot \vec{S}_1 \vec{v}_1 \cdot \vec{v}_2 \right) \log \left( \frac{r}{R_0} \right) + \\
& \frac{1}{\epsilon_d} \left( \frac{-\frac{4}{7} \hat{n} \cdot \vec{S}_1 \hat{n} \cdot \vec{S}_1 \hat{n} \cdot \vec{v}_1 + \frac{4}{35} \vec{S}_1 \cdot \vec{S}_1 \hat{n} \cdot \vec{v}_1 + \frac{4}{35} \hat{n} \cdot \vec{S}_1 \vec{S}_1 \cdot \vec{v}_1 + \frac{4}{35} \hat{n} \cdot \vec{S}_1 \vec{S}_1 \cdot \vec{v}_1}{r^4} + \frac{1}{r^5} \right. \\
& \left( \frac{7}{4} (\hat{n} \cdot \vec{v}_1)^2 (\hat{n} \cdot \vec{S}_1)^2 - 2 \hat{n} \cdot \vec{v}_1 \hat{n} \cdot \vec{v}_2 (\hat{n} \cdot \vec{S}_1)^2 - \frac{1}{4} \vec{v}_1 \cdot \vec{v}_1 (\hat{n} \cdot \vec{S}_1)^2 + \frac{2}{7} \vec{v}_1 \cdot \vec{v}_2 (\hat{n} \cdot \vec{S}_1)^2 - \right. \\
& \hat{n} \cdot \vec{v}_1 \vec{S}_1 \cdot \vec{v}_1 \hat{n} \cdot \vec{S}_1 + \frac{4}{7} \hat{n} \cdot \vec{v}_2 \vec{S}_1 \cdot \vec{v}_1 \hat{n} \cdot \vec{S}_1 + \frac{4}{7} \hat{n} \cdot \vec{v}_1 \vec{S}_1 \cdot \vec{v}_2 \hat{n} \cdot \vec{S}_1 + \frac{1}{10} (\vec{S}_1 \cdot \vec{v}_1)^2 - \frac{1}{4} (\hat{n} \cdot \vec{v}_1)^2 \vec{S}_1 \cdot \vec{S}_1 + \\
& \left. \frac{2}{7} \hat{n} \cdot \vec{v}_1 \hat{n} \cdot \vec{v}_2 \vec{S}_1 \cdot \vec{S}_1 - \frac{4}{35} \vec{S}_1 \cdot \vec{v}_1 \vec{S}_1 \cdot \vec{v}_2 + \frac{1}{20} \vec{S}_1 \cdot \vec{S}_1 \vec{v}_1 \cdot \vec{v}_1 - \frac{2}{35} \vec{S}_1 \cdot \vec{S}_1 \vec{v}_1 \cdot \vec{v}_2 \right) \left. \right) \Bigg\} c_{\text{ES}^2 1} \Bigg\}
\end{aligned}$$

{DiagS1CES2[3, 1, 45],

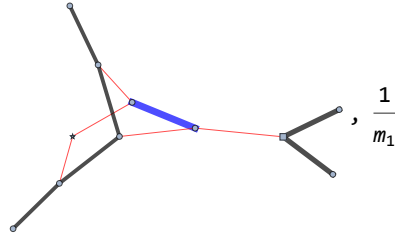

$$\begin{aligned}
& G^3 m_2^3 \left( \frac{\frac{64}{3} \hat{n} \cdot \vec{S}_1 \hat{n} \cdot \vec{S}_1 \hat{n} \cdot \vec{v}_2 - \frac{20}{3} \vec{S}_1 \cdot \vec{S}_1 \hat{n} \cdot \vec{v}_2 - \frac{11}{3} \hat{n} \cdot \vec{S}_1 \vec{S}_1 \cdot \vec{v}_2 - \frac{11}{3} \hat{n} \cdot \vec{S}_1 \vec{S}_1 \cdot \vec{v}_2}{r^4} + \frac{1}{r^5} \right. \\
& \left( \frac{523}{6} (\hat{n} \cdot \vec{v}_2)^2 (\hat{n} \cdot \vec{S}_1)^2 - \frac{493}{6} \hat{n} \cdot \vec{v}_1 \hat{n} \cdot \vec{v}_2 (\hat{n} \cdot \vec{S}_1)^2 + \frac{32}{3} \vec{v}_1 \cdot \vec{v}_2 (\hat{n} \cdot \vec{S}_1)^2 - \frac{79}{6} \vec{v}_2 \cdot \vec{v}_2 (\hat{n} \cdot \vec{S}_1)^2 + \right. \\
& \frac{64}{3} \hat{n} \cdot \vec{v}_2 \vec{S}_1 \cdot \vec{v}_1 \hat{n} \cdot \vec{S}_1 + \frac{64}{3} \hat{n} \cdot \vec{v}_1 \vec{S}_1 \cdot \vec{v}_2 \hat{n} \cdot \vec{S}_1 - \frac{134}{3} \hat{n} \cdot \vec{v}_2 \vec{S}_1 \cdot \vec{v}_2 \hat{n} \cdot \vec{S}_1 + \frac{281}{75} (\vec{S}_1 \cdot \vec{v}_2)^2 - \\
& \frac{121}{6} (\hat{n} \cdot \vec{v}_2)^2 \vec{S}_1 \cdot \vec{S}_1 + \frac{109}{6} \hat{n} \cdot \vec{v}_1 \hat{n} \cdot \vec{v}_2 \vec{S}_1 \cdot \vec{S}_1 - \frac{11}{3} \vec{S}_1 \cdot \vec{v}_1 \vec{S}_1 \cdot \vec{v}_2 - \frac{10}{3} \vec{S}_1 \cdot \vec{S}_1 \vec{v}_1 \cdot \vec{v}_2 + \frac{731}{150} \vec{S}_1 \cdot \vec{S}_1 \vec{v}_2 \cdot \vec{v}_2 \Bigg) + \\
& \left( \frac{-15 \hat{n} \cdot \vec{S}_1 \hat{n} \cdot \vec{S}_1 \hat{n} \cdot \vec{v}_2 + 3 \vec{S}_1 \cdot \vec{S}_1 \hat{n} \cdot \vec{v}_2 + 3 \hat{n} \cdot \vec{S}_1 \vec{S}_1 \cdot \vec{v}_2 + 3 \hat{n} \cdot \vec{S}_1 \vec{S}_1 \cdot \vec{v}_2}{r^4} + \frac{1}{r^5} \right. \\
& \left( -63 (\hat{n} \cdot \vec{v}_2)^2 (\hat{n} \cdot \vec{S}_1)^2 + \frac{105}{2} \hat{n} \cdot \vec{v}_1 \hat{n} \cdot \vec{v}_2 (\hat{n} \cdot \vec{S}_1)^2 - \frac{15}{2} \vec{v}_1 \cdot \vec{v}_2 (\hat{n} \cdot \vec{S}_1)^2 + 9 \vec{v}_2 \cdot \vec{v}_2 (\hat{n} \cdot \vec{S}_1)^2 - \right.
\end{aligned}$$



$$\begin{aligned}
& 15 \hat{n} \cdot \vec{v}_2 \vec{S}_1 \cdot \vec{v}_1 \hat{n} \cdot \vec{S}_1 - 15 \hat{n} \cdot \vec{v}_1 \vec{S}_1 \cdot \vec{v}_2 \hat{n} \cdot \vec{S}_1 + 36 \hat{n} \cdot \vec{v}_2 \vec{S}_1 \cdot \vec{v}_2 \hat{n} \cdot \vec{S}_1 - \frac{18}{5} (\vec{S}_1 \cdot \vec{v}_2)^2 + 9 (\hat{n} \cdot \vec{v}_2)^2 \vec{S}_1 \cdot \vec{S}_1 - \\
& \frac{15}{2} \hat{n} \cdot \vec{v}_1 \hat{n} \cdot \vec{v}_2 \vec{S}_1 \cdot \vec{S}_1 + 3 \vec{S}_1 \cdot \vec{v}_1 \vec{S}_1 \cdot \vec{v}_2 + \frac{3}{2} \vec{S}_1 \cdot \vec{S}_1 \vec{v}_1 \cdot \vec{v}_2 - \frac{9}{5} \vec{S}_1 \cdot \vec{S}_1 \vec{v}_2 \cdot \vec{v}_2 \left) \log \left( \frac{r}{R_\theta} \right) + \right. \\
& \frac{1}{\epsilon_d} \left( \frac{5 \hat{n} \cdot \vec{S}_1 \hat{n} \cdot \vec{S}_1 \hat{n} \cdot \vec{v}_2 - \vec{S}_1 \cdot \vec{S}_1 \hat{n} \cdot \vec{v}_2 - \hat{n} \cdot \vec{S}_1 \vec{S}_1 \cdot \vec{v}_2 - \hat{n} \cdot \vec{S}_1 \vec{S}_1 \cdot \vec{v}_2}{r^4} + \frac{1}{r^5} \right. \\
& \left( 21 (\hat{n} \cdot \vec{v}_2)^2 (\hat{n} \cdot \vec{S}_1)^2 - \frac{35}{2} \hat{n} \cdot \vec{v}_1 \hat{n} \cdot \vec{v}_2 (\hat{n} \cdot \vec{S}_1)^2 + \frac{5}{2} \vec{v}_1 \cdot \vec{v}_2 (\hat{n} \cdot \vec{S}_1)^2 - 3 \vec{v}_2 \cdot \vec{v}_2 (\hat{n} \cdot \vec{S}_1)^2 + \right. \\
& 5 \hat{n} \cdot \vec{v}_2 \vec{S}_1 \cdot \vec{v}_1 \hat{n} \cdot \vec{S}_1 + 5 \hat{n} \cdot \vec{v}_1 \vec{S}_1 \cdot \vec{v}_2 \hat{n} \cdot \vec{S}_1 - 12 \hat{n} \cdot \vec{v}_2 \vec{S}_1 \cdot \vec{v}_2 \hat{n} \cdot \vec{S}_1 + \frac{6}{5} (\vec{S}_1 \cdot \vec{v}_2)^2 - 3 (\hat{n} \cdot \vec{v}_2)^2 \vec{S}_1 \cdot \vec{S}_1 + \\
& \left. \left. \frac{5}{2} \hat{n} \cdot \vec{v}_1 \hat{n} \cdot \vec{v}_2 \vec{S}_1 \cdot \vec{S}_1 - \vec{S}_1 \cdot \vec{v}_1 \vec{S}_1 \cdot \vec{v}_2 - \frac{1}{2} \vec{S}_1 \cdot \vec{S}_1 \vec{v}_1 \cdot \vec{v}_2 + \frac{3}{5} \vec{S}_1 \cdot \vec{S}_1 \vec{v}_2 \cdot \vec{v}_2 \right) \right) \left. \right) \Bigg\} c_{\text{ES}^2_1}
\end{aligned}$$

$$\left\{ \text{DiagS1CES2}[3, 1, 46], \frac{1}{m_1} \right\}$$
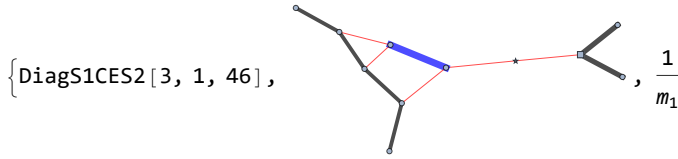

$$\begin{aligned}
& G^3 m_2^3 \left( \frac{\frac{23}{2} \hat{n} \cdot \vec{S}_1 \hat{n} \cdot \vec{S}_1 \hat{n} \cdot \vec{v}_2 - \frac{7}{2} \vec{S}_1 \cdot \vec{S}_1 \hat{n} \cdot \vec{v}_2 - 2 \hat{n} \cdot \vec{S}_1 \vec{S}_1 \cdot \vec{v}_2 - 2 \hat{n} \cdot \vec{S}_1 \vec{S}_1 \cdot \vec{v}_2}{r^4} + \right. \\
& \frac{1}{r^5} \left( -44 \hat{n} \cdot \vec{v}_1 \hat{n} \cdot \vec{v}_2 (\hat{n} \cdot \vec{S}_1)^2 + \frac{23}{4} \vec{v}_1 \cdot \vec{v}_2 (\hat{n} \cdot \vec{S}_1)^2 + \frac{23}{2} \hat{n} \cdot \vec{v}_2 \vec{S}_1 \cdot \vec{v}_1 \hat{n} \cdot \vec{S}_1 + \right. \\
& \frac{23}{2} \hat{n} \cdot \vec{v}_1 \vec{S}_1 \cdot \vec{v}_2 \hat{n} \cdot \vec{S}_1 + \frac{19}{2} \hat{n} \cdot \vec{v}_1 \hat{n} \cdot \vec{v}_2 \vec{S}_1 \cdot \vec{S}_1 - 2 \vec{S}_1 \cdot \vec{v}_1 \vec{S}_1 \cdot \vec{v}_2 - \frac{7}{4} \vec{S}_1 \cdot \vec{S}_1 \vec{v}_1 \cdot \vec{v}_2 \Big) + \\
& \left( \frac{-\frac{15}{2} \hat{n} \cdot \vec{S}_1 \hat{n} \cdot \vec{S}_1 \hat{n} \cdot \vec{v}_2 + \frac{3}{2} \vec{S}_1 \cdot \vec{S}_1 \hat{n} \cdot \vec{v}_2 + \frac{3}{2} \hat{n} \cdot \vec{S}_1 \vec{S}_1 \cdot \vec{v}_2 + \frac{3}{2} \hat{n} \cdot \vec{S}_1 \vec{S}_1 \cdot \vec{v}_2}{r^4} + \frac{1}{r^5} \right. \\
& \left( \frac{105}{4} \hat{n} \cdot \vec{v}_1 \hat{n} \cdot \vec{v}_2 (\hat{n} \cdot \vec{S}_1)^2 - \frac{15}{4} \vec{v}_1 \cdot \vec{v}_2 (\hat{n} \cdot \vec{S}_1)^2 - \frac{15}{2} \hat{n} \cdot \vec{v}_2 \vec{S}_1 \cdot \vec{v}_1 \hat{n} \cdot \vec{S}_1 - \right. \\
& \frac{15}{2} \hat{n} \cdot \vec{v}_1 \vec{S}_1 \cdot \vec{v}_2 \hat{n} \cdot \vec{S}_1 - \frac{15}{4} \hat{n} \cdot \vec{v}_1 \hat{n} \cdot \vec{v}_2 \vec{S}_1 \cdot \vec{S}_1 + \frac{3}{2} \vec{S}_1 \cdot \vec{v}_1 \vec{S}_1 \cdot \vec{v}_2 + \frac{3}{4} \vec{S}_1 \cdot \vec{S}_1 \vec{v}_1 \cdot \vec{v}_2 \Big) \log \left( \frac{r}{R_\theta} \right) + \\
& \frac{1}{\epsilon_d} \left( \frac{\frac{5}{2} \hat{n} \cdot \vec{S}_1 \hat{n} \cdot \vec{S}_1 \hat{n} \cdot \vec{v}_2 - \frac{1}{2} \vec{S}_1 \cdot \vec{S}_1 \hat{n} \cdot \vec{v}_2 - \frac{1}{2} \hat{n} \cdot \vec{S}_1 \vec{S}_1 \cdot \vec{v}_2 - \frac{1}{2} \hat{n} \cdot \vec{S}_1 \vec{S}_1 \cdot \vec{v}_2}{r^4} + \frac{1}{r^5} \right. \\
& \left( -\frac{35}{4} \hat{n} \cdot \vec{v}_1 \hat{n} \cdot \vec{v}_2 (\hat{n} \cdot \vec{S}_1)^2 + \frac{5}{4} \vec{v}_1 \cdot \vec{v}_2 (\hat{n} \cdot \vec{S}_1)^2 + \frac{5}{2} \hat{n} \cdot \vec{v}_2 \vec{S}_1 \cdot \vec{v}_1 \hat{n} \cdot \vec{S}_1 + \right. \\
& \frac{5}{2} \hat{n} \cdot \vec{v}_1 \vec{S}_1 \cdot \vec{v}_2 \hat{n} \cdot \vec{S}_1 + \frac{5}{4} \hat{n} \cdot \vec{v}_1 \hat{n} \cdot \vec{v}_2 \vec{S}_1 \cdot \vec{S}_1 - \frac{1}{2} \vec{S}_1 \cdot \vec{v}_1 \vec{S}_1 \cdot \vec{v}_2 - \frac{1}{4} \vec{S}_1 \cdot \vec{S}_1 \vec{v}_1 \cdot \vec{v}_2 \Big) \Bigg\} c_{\text{ES}^2_1}
\end{aligned}$$

{DiagS1CES2[3, 1, 47],

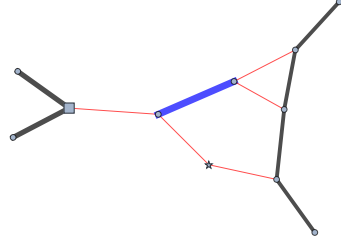

$$, \frac{1}{m_1} G^3 m_2^3 C_{\text{ES}^2 1}$$

$$\left( \frac{\frac{7}{4} (\hat{n} \cdot \vec{S}_1)^2 (\hat{n} \cdot \vec{v}_2)^2 - \frac{1}{4} \vec{v}_2 \cdot \vec{v}_2 (\hat{n} \cdot \vec{S}_1)^2 - \hat{n} \cdot \vec{S}_1 \hat{n} \cdot \vec{v}_2 \vec{S}_1 \cdot \vec{v}_2 - \frac{1}{4} \vec{S}_1 \cdot \vec{S}_1 (\hat{n} \cdot \vec{v}_2)^2 + \frac{1}{10} (\vec{S}_1 \cdot \vec{v}_2)^2 + \frac{1}{20} \vec{S}_1 \cdot \vec{S}_1 \vec{v}_2 \cdot \vec{v}_2}{r^5 \in_d} + \right.$$

$$\frac{1}{r^5} \log \left( \frac{r}{R_0} \right) \left( -\frac{21}{4} (\hat{n} \cdot \vec{S}_1)^2 (\hat{n} \cdot \vec{v}_2)^2 + \frac{3}{4} \vec{v}_2 \cdot \vec{v}_2 (\hat{n} \cdot \vec{S}_1)^2 + 3 \hat{n} \cdot \vec{S}_1 \hat{n} \cdot \vec{v}_2 \vec{S}_1 \cdot \vec{v}_2 + \frac{3}{4} \vec{S}_1 \cdot \vec{S}_1 (\hat{n} \cdot \vec{v}_2)^2 - \right.$$

$$\frac{3}{10} (\vec{S}_1 \cdot \vec{v}_2)^2 - \frac{3}{20} \vec{S}_1 \cdot \vec{S}_1 \vec{v}_2 \cdot \vec{v}_2 \Big) + \frac{1}{r^5} \left( \frac{41}{8} (\hat{n} \cdot \vec{S}_1)^2 (\hat{n} \cdot \vec{v}_2)^2 + \frac{35}{4} (\hat{n} \cdot \vec{S}_1)^2 \hat{n} \cdot \vec{v}_1 \hat{n} \cdot \vec{v}_2 - \frac{5}{4} \vec{v}_1 \cdot \vec{v}_2 (\hat{n} \cdot \vec{S}_1)^2 - \right.$$

$$\frac{13}{8} \vec{v}_2 \cdot \vec{v}_2 (\hat{n} \cdot \vec{S}_1)^2 - \frac{5}{2} \hat{n} \cdot \vec{S}_1 \hat{n} \cdot \vec{v}_2 \vec{S}_1 \cdot \vec{v}_1 - \frac{5}{2} \hat{n} \cdot \vec{S}_1 \hat{n} \cdot \vec{v}_1 \vec{S}_1 \cdot \vec{v}_2 - \frac{5}{2} \hat{n} \cdot \vec{S}_1 \hat{n} \cdot \vec{v}_2 \vec{S}_1 \cdot \vec{v}_2 - \frac{11}{8} \vec{S}_1 \cdot \vec{S}_1 (\hat{n} \cdot \vec{v}_2)^2 -$$

$$\frac{5}{4} \vec{S}_1 \cdot \vec{S}_1 \hat{n} \cdot \vec{v}_1 \hat{n} \cdot \vec{v}_2 + \frac{19}{100} (\vec{S}_1 \cdot \vec{v}_2)^2 + \frac{1}{2} \vec{S}_1 \cdot \vec{v}_1 \vec{S}_1 \cdot \vec{v}_2 + \frac{1}{4} \vec{S}_1 \cdot \vec{S}_1 \vec{v}_1 \cdot \vec{v}_2 + \frac{169}{200} \vec{S}_1 \cdot \vec{S}_1 \vec{v}_2 \cdot \vec{v}_2 \Big) +$$

$$\left. \frac{-\frac{5}{2} \hat{n} \cdot \vec{S}_1 \hat{n} \cdot \vec{S}_1 \hat{n} \cdot \vec{v}_2 + \frac{1}{2} \vec{S}_1 \cdot \vec{S}_1 \hat{n} \cdot \vec{v}_2 + \frac{1}{2} \hat{n} \cdot \vec{S}_1 \vec{S}_1 \cdot \vec{v}_2 + \frac{1}{2} \hat{n} \cdot \vec{S}_1 \vec{S}_1 \cdot \vec{v}_2}{r^4} \right\}$$

{DiagS1CES2[3, 1, 48],

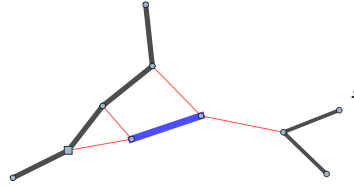

$$G^3 m_1 m_2 \left( \frac{\frac{110}{49} \hat{n} \cdot \vec{S}_1 \hat{n} \cdot \vec{S}_1 \hat{n} \cdot \vec{v}_1 - \frac{1467 \vec{S}_1 \cdot \vec{S}_1 \hat{n} \cdot \vec{v}_1}{1225} - \frac{519 \hat{n} \cdot \vec{S}_1 \vec{S}_1 \cdot \vec{v}_1}{2450} + \frac{2}{5} \hat{n} \cdot \vec{S}_1 \vec{S}_1 \cdot \vec{a}_1 - \frac{519 \hat{n} \cdot \vec{S}_1 \vec{S}_1 \cdot \vec{v}_1}{2450}}{r^4} + \frac{1}{r^5} \right.$$

$$\left( -\frac{109}{24} (\hat{n} \cdot \vec{v}_1)^2 (\hat{n} \cdot \vec{S}_1)^2 + 5 \hat{n} \cdot \vec{v}_1 \hat{n} \cdot \vec{v}_2 (\hat{n} \cdot \vec{S}_1)^2 - \frac{1285 \vec{v}_1 \cdot \vec{v}_1 (\hat{n} \cdot \vec{S}_1)^2}{1176} - \frac{61}{98} \vec{v}_1 \cdot \vec{v}_2 (\hat{n} \cdot \vec{S}_1)^2 - \right.$$

$$\frac{9}{14} \vec{v}_2 \cdot \vec{v}_2 (\hat{n} \cdot \vec{S}_1)^2 + \frac{941}{294} \hat{n} \cdot \vec{v}_1 \vec{S}_1 \cdot \vec{v}_1 \hat{n} \cdot \vec{S}_1 - \frac{40}{49} \hat{n} \cdot \vec{v}_2 \vec{S}_1 \cdot \vec{v}_1 \hat{n} \cdot \vec{S}_1 - \frac{61}{49} \hat{n} \cdot \vec{v}_1 \vec{S}_1 \cdot \vec{v}_2 \hat{n} \cdot \vec{S}_1 - \frac{275}{588} (\vec{S}_1 \cdot \vec{v}_1)^2 +$$

$$\frac{283 (\hat{n} \cdot \vec{v}_1)^2 \vec{S}_1 \cdot \vec{S}_1}{1176} - \frac{55}{49} \hat{n} \cdot \vec{v}_1 \hat{n} \cdot \vec{v}_2 \vec{S}_1 \cdot \vec{S}_1 + \frac{137 \vec{S}_1 \cdot \vec{v}_1 \vec{S}_1 \cdot \vec{v}_2}{1225} + \frac{235}{392} \vec{S}_1 \cdot \vec{S}_1 \vec{v}_1 \cdot \vec{v}_1 + \frac{487 \vec{S}_1 \cdot \vec{S}_1 \vec{v}_1 \cdot \vec{v}_2}{2450} +$$

$$\frac{3}{14} \vec{S}_1 \cdot \vec{S}_1 \vec{v}_2 \cdot \vec{v}_2 \Big) + \left( \frac{-\frac{9}{7} \hat{n} \cdot \vec{S}_1 \hat{n} \cdot \vec{S}_1 \hat{n} \cdot \vec{v}_1 + \frac{9}{35} \vec{S}_1 \cdot \vec{S}_1 \hat{n} \cdot \vec{v}_1 + \frac{9}{35} \hat{n} \cdot \vec{S}_1 \vec{S}_1 \cdot \vec{v}_1 + \frac{9}{35} \hat{n} \cdot \vec{S}_1 \vec{S}_1 \cdot \vec{v}_1}{r^4} + \right.$$

$$\frac{1}{r^5} \left( \frac{5}{2} (\hat{n} \cdot \vec{v}_1)^2 (\hat{n} \cdot \vec{S}_1)^2 - \frac{9}{2} \hat{n} \cdot \vec{v}_1 \hat{n} \cdot \vec{v}_2 (\hat{n} \cdot \vec{S}_1)^2 - \frac{5}{14} \vec{v}_1 \cdot \vec{v}_1 (\hat{n} \cdot \vec{S}_1)^2 + \frac{9}{14} \vec{v}_1 \cdot \vec{v}_2 (\hat{n} \cdot \vec{S}_1)^2 - \right.$$

$$\frac{10}{7} \hat{n} \cdot \vec{v}_1 \vec{S}_1 \cdot \vec{v}_1 \hat{n} \cdot \vec{S}_1 + \frac{9}{7} \hat{n} \cdot \vec{v}_2 \vec{S}_1 \cdot \vec{v}_1 \hat{n} \cdot \vec{S}_1 + \frac{9}{7} \hat{n} \cdot \vec{v}_1 \vec{S}_1 \cdot \vec{v}_2 \hat{n} \cdot \vec{S}_1 + \frac{1}{7} (\vec{S}_1 \cdot \vec{v}_1)^2 - \frac{5}{14} (\hat{n} \cdot \vec{v}_1)^2 \vec{S}_1 \cdot \vec{S}_1 +$$

$$\begin{aligned}
& \left. \frac{9}{14} \hat{n} \cdot \vec{v}_1 \hat{n} \cdot \vec{v}_2 \vec{S}_1 \cdot \vec{S}_1 - \frac{9}{35} \vec{S}_1 \cdot \vec{v}_1 \vec{S}_1 \cdot \vec{v}_2 + \frac{1}{14} \vec{S}_1 \cdot \vec{S}_1 \vec{v}_1 \cdot \vec{v}_1 - \frac{9}{70} \vec{S}_1 \cdot \vec{S}_1 \vec{v}_1 \cdot \vec{v}_2 \right) \log \left( \frac{r}{R_\theta} \right) + \\
& \frac{2 \vec{S}_1^2}{3 r^3} + \frac{1}{\epsilon_d} \left( \frac{\frac{3}{7} \hat{n} \cdot \vec{S}_1 \hat{n} \cdot \vec{S}_1 \hat{n} \cdot \vec{v}_1 - \frac{3}{35} \vec{S}_1 \cdot \vec{S}_1 \hat{n} \cdot \vec{v}_1 - \frac{3}{35} \hat{n} \cdot \vec{S}_1 \vec{S}_1 \cdot \vec{v}_1 - \frac{3}{35} \hat{n} \cdot \vec{S}_1 \vec{S}_1 \cdot \vec{v}_1}{r^4} + \frac{1}{r^5} \right. \\
& \left( -\frac{5}{6} (\hat{n} \cdot \vec{v}_1)^2 (\hat{n} \cdot \vec{S}_1)^2 + \frac{3}{2} \hat{n} \cdot \vec{v}_1 \hat{n} \cdot \vec{v}_2 (\hat{n} \cdot \vec{S}_1)^2 + \frac{5}{42} \vec{v}_1 \cdot \vec{v}_1 (\hat{n} \cdot \vec{S}_1)^2 - \frac{3}{14} \vec{v}_1 \cdot \vec{v}_2 (\hat{n} \cdot \vec{S}_1)^2 + \right. \\
& \frac{10}{21} \hat{n} \cdot \vec{v}_1 \vec{S}_1 \cdot \vec{v}_1 \hat{n} \cdot \vec{S}_1 - \frac{3}{7} \hat{n} \cdot \vec{v}_2 \vec{S}_1 \cdot \vec{v}_1 \hat{n} \cdot \vec{S}_1 - \frac{3}{7} \hat{n} \cdot \vec{v}_1 \vec{S}_1 \cdot \vec{v}_2 \hat{n} \cdot \vec{S}_1 - \frac{1}{21} (\vec{S}_1 \cdot \vec{v}_1)^2 + \frac{5}{42} (\hat{n} \cdot \vec{v}_1)^2 \vec{S}_1 \cdot \vec{S}_1 - \\
& \left. \left. \frac{3}{14} \hat{n} \cdot \vec{v}_1 \hat{n} \cdot \vec{v}_2 \vec{S}_1 \cdot \vec{S}_1 + \frac{3}{35} \vec{S}_1 \cdot \vec{v}_1 \vec{S}_1 \cdot \vec{v}_2 - \frac{1}{42} \vec{S}_1 \cdot \vec{S}_1 \vec{v}_1 \cdot \vec{v}_1 + \frac{3}{70} \vec{S}_1 \cdot \vec{S}_1 \vec{v}_1 \cdot \vec{v}_2 \right) \right) \left. \right\} C_{ES^2_1} \}
\end{aligned}$$

{DiagS1CES2[3, 1, 49],

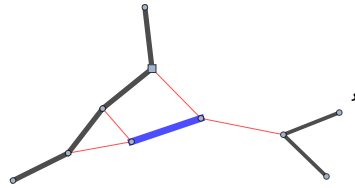

$$\begin{aligned}
& G^3 m_1 m_2 \left( \frac{1}{r^4} \left( -\frac{7}{2} \hat{n} \cdot \vec{S}_1 \hat{n} \cdot \vec{S}_1 \hat{n} \cdot \vec{v}_2 + \frac{51}{50} \vec{S}_1 \cdot \vec{S}_1 \hat{n} \cdot \vec{v}_2 + \frac{3}{5} \hat{n} \cdot \vec{S}_1 \vec{S}_1 \cdot \vec{v}_1 + \right. \right. \\
& \frac{13}{25} \hat{n} \cdot \vec{S}_1 \vec{S}_1 \cdot \vec{v}_2 - \frac{6}{5} \hat{n} \cdot \vec{v}_1 \vec{S}_1 \cdot \vec{S}_1 + \frac{3}{5} \hat{n} \cdot \vec{S}_1 \vec{S}_1 \cdot \vec{a}_1 + \frac{3}{5} \hat{n} \cdot \vec{S}_1 \vec{S}_1 \cdot \vec{v}_1 + \frac{13}{25} \hat{n} \cdot \vec{S}_1 \vec{S}_1 \cdot \vec{v}_2 \left. \right) + \frac{1}{r^5} \\
& \left( -\frac{17}{24} (\hat{n} \cdot \vec{v}_1)^2 (\hat{n} \cdot \vec{S}_1)^2 + \frac{19}{2} \hat{n} \cdot \vec{v}_1 \hat{n} \cdot \vec{v}_2 (\hat{n} \cdot \vec{S}_1)^2 - \frac{2109}{392} \vec{v}_1 \cdot \vec{v}_1 (\hat{n} \cdot \vec{S}_1)^2 - \frac{221}{196} \vec{v}_1 \cdot \vec{v}_2 (\hat{n} \cdot \vec{S}_1)^2 - \right. \\
& \frac{27}{14} \vec{v}_2 \cdot \vec{v}_2 (\hat{n} \cdot \vec{S}_1)^2 + \frac{69}{49} \hat{n} \cdot \vec{v}_1 \vec{S}_1 \cdot \vec{v}_1 \hat{n} \cdot \vec{S}_1 - \frac{263}{98} \hat{n} \cdot \vec{v}_2 \vec{S}_1 \cdot \vec{v}_1 \hat{n} \cdot \vec{S}_1 - \\
& \frac{221}{98} \hat{n} \cdot \vec{v}_1 \vec{S}_1 \cdot \vec{v}_2 \hat{n} \cdot \vec{S}_1 - \frac{6403 (\vec{S}_1 \cdot \vec{v}_1)^2}{14700} - \frac{1273 (\hat{n} \cdot \vec{v}_1)^2 \vec{S}_1 \cdot \vec{S}_1}{1176} - \frac{92}{49} \hat{n} \cdot \vec{v}_1 \hat{n} \cdot \vec{v}_2 \vec{S}_1 \cdot \vec{S}_1 + \\
& \left. \frac{20}{49} \vec{S}_1 \cdot \vec{v}_1 \vec{S}_1 \cdot \vec{v}_2 + \frac{65347 \vec{S}_1 \cdot \vec{S}_1 \vec{v}_1 \cdot \vec{v}_1}{29400} + \frac{61}{196} \vec{S}_1 \cdot \vec{S}_1 \vec{v}_1 \cdot \vec{v}_2 + \frac{9}{14} \vec{S}_1 \cdot \vec{S}_1 \vec{v}_2 \cdot \vec{v}_2 \right) + \\
& \left( \frac{\frac{9}{2} \hat{n} \cdot \vec{S}_1 \hat{n} \cdot \vec{S}_1 \hat{n} \cdot \vec{v}_2 - \frac{9}{10} \vec{S}_1 \cdot \vec{S}_1 \hat{n} \cdot \vec{v}_2 - \frac{9}{10} \hat{n} \cdot \vec{S}_1 \vec{S}_1 \cdot \vec{v}_2 - \frac{9}{10} \hat{n} \cdot \vec{S}_1 \vec{S}_1 \cdot \vec{v}_2}{r^4} + \frac{1}{r^5} \right. \\
& \left( \frac{1}{4} (\hat{n} \cdot \vec{v}_1)^2 (\hat{n} \cdot \vec{S}_1)^2 - \frac{45}{4} \hat{n} \cdot \vec{v}_1 \hat{n} \cdot \vec{v}_2 (\hat{n} \cdot \vec{S}_1)^2 - \frac{1}{28} \vec{v}_1 \cdot \vec{v}_1 (\hat{n} \cdot \vec{S}_1)^2 + \frac{45}{28} \vec{v}_1 \cdot \vec{v}_2 (\hat{n} \cdot \vec{S}_1)^2 - \right. \\
& \frac{1}{7} \hat{n} \cdot \vec{v}_1 \vec{S}_1 \cdot \vec{v}_1 \hat{n} \cdot \vec{S}_1 + \frac{45}{14} \hat{n} \cdot \vec{v}_2 \vec{S}_1 \cdot \vec{v}_1 \hat{n} \cdot \vec{S}_1 + \frac{45}{14} \hat{n} \cdot \vec{v}_1 \vec{S}_1 \cdot \vec{v}_2 \hat{n} \cdot \vec{S}_1 + \frac{1}{70} (\vec{S}_1 \cdot \vec{v}_1)^2 - \frac{1}{28} (\hat{n} \cdot \vec{v}_1)^2 \vec{S}_1 \cdot \vec{S}_1 + \\
& \left. \left. \frac{45}{28} \hat{n} \cdot \vec{v}_1 \hat{n} \cdot \vec{v}_2 \vec{S}_1 \cdot \vec{S}_1 - \frac{9}{14} \vec{S}_1 \cdot \vec{v}_1 \vec{S}_1 \cdot \vec{v}_2 + \frac{1}{140} \vec{S}_1 \cdot \vec{S}_1 \vec{v}_1 \cdot \vec{v}_1 - \frac{9}{28} \vec{S}_1 \cdot \vec{S}_1 \vec{v}_1 \cdot \vec{v}_2 \right) \right) \log \left( \frac{r}{R_\theta} \right) +
\end{aligned}$$

$$\frac{\vec{S}_1^2}{3r^3} + \frac{1}{\epsilon_d} \left( \frac{-\frac{3}{2} \hat{n} \cdot \vec{S}_1 \hat{n} \cdot \vec{S}_1 \hat{n} \cdot \vec{v}_2 + \frac{3}{10} \vec{S}_1 \cdot \vec{S}_1 \hat{n} \cdot \vec{v}_2 + \frac{3}{10} \hat{n} \cdot \vec{S}_1 \vec{S}_1 \cdot \vec{v}_2 + \frac{3}{10} \hat{n} \cdot \vec{S}_1 \vec{S}_1 \cdot \vec{v}_2}{r^4} + \frac{1}{r^5} \right. \\ \left( -\frac{1}{12} (\hat{n} \cdot \vec{v}_1)^2 (\hat{n} \cdot \vec{S}_1)^2 + \frac{15}{4} \hat{n} \cdot \vec{v}_1 \hat{n} \cdot \vec{v}_2 (\hat{n} \cdot \vec{S}_1)^2 + \frac{1}{84} \vec{v}_1 \cdot \vec{v}_1 (\hat{n} \cdot \vec{S}_1)^2 - \frac{15}{28} \vec{v}_1 \cdot \vec{v}_2 (\hat{n} \cdot \vec{S}_1)^2 + \right. \\ \left. \frac{1}{21} \hat{n} \cdot \vec{v}_1 \vec{S}_1 \cdot \vec{v}_1 \hat{n} \cdot \vec{S}_1 - \frac{15}{14} \hat{n} \cdot \vec{v}_2 \vec{S}_1 \cdot \vec{v}_1 \hat{n} \cdot \vec{S}_1 - \frac{15}{14} \hat{n} \cdot \vec{v}_1 \vec{S}_1 \cdot \vec{v}_2 \hat{n} \cdot \vec{S}_1 - \frac{1}{210} (\vec{S}_1 \cdot \vec{v}_1)^2 + \frac{1}{84} (\hat{n} \cdot \vec{v}_1)^2 \vec{S}_1 \cdot \vec{S}_1 - \right. \\ \left. \frac{15}{28} \hat{n} \cdot \vec{v}_1 \hat{n} \cdot \vec{v}_2 \vec{S}_1 \cdot \vec{S}_1 + \frac{3}{14} \vec{S}_1 \cdot \vec{v}_1 \vec{S}_1 \cdot \vec{v}_2 - \frac{1}{420} \vec{S}_1 \cdot \vec{S}_1 \vec{v}_1 \cdot \vec{v}_1 + \frac{3}{28} \vec{S}_1 \cdot \vec{S}_1 \vec{v}_1 \cdot \vec{v}_2 \right) \Bigg) \Bigg\} c_{\text{ES}^2 1}$$

{DiagS1CES2[3, 1, 50], 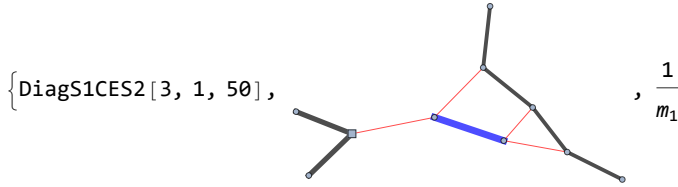 ,  $\frac{1}{m_1}$

$$G^3 m_2^3 \left( \frac{1}{r^4} \left( -\frac{13}{2} \hat{n} \cdot \vec{S}_1 \hat{n} \cdot \vec{S}_1 \hat{n} \cdot \vec{v}_2 + \frac{5}{2} \vec{S}_1 \cdot \vec{S}_1 \hat{n} \cdot \vec{v}_2 + \hat{n} \cdot \vec{S}_1 \vec{S}_1 \cdot \vec{v}_1 + \hat{n} \cdot \vec{S}_1 \vec{S}_1 \cdot \vec{v}_2 - 2 \hat{n} \cdot \vec{v}_1 \vec{S}_1 \cdot \vec{S}_1 + \hat{n} \cdot \vec{S}_1 \vec{S}_1 \cdot \vec{a}_1 + \right. \right. \\ \left. \hat{n} \cdot \vec{S}_1 \vec{S}_1 \cdot \vec{v}_1 + \hat{n} \cdot \vec{S}_1 \vec{S}_1 \cdot \vec{v}_2 \right) + \frac{1}{r^5} \left( -\frac{83}{8} (\hat{n} \cdot \vec{v}_2)^2 (\hat{n} \cdot \vec{S}_1)^2 + \frac{53}{2} \hat{n} \cdot \vec{v}_1 \hat{n} \cdot \vec{v}_2 (\hat{n} \cdot \vec{S}_1)^2 - \frac{15}{4} \vec{v}_1 \cdot \vec{v}_1 (\hat{n} \cdot \vec{S}_1)^2 - \right. \\ \left. \frac{13}{4} \vec{v}_1 \cdot \vec{v}_2 (\hat{n} \cdot \vec{S}_1)^2 - \frac{71}{8} \vec{v}_2 \cdot \vec{v}_2 (\hat{n} \cdot \vec{S}_1)^2 + \frac{5}{2} \hat{n} \cdot \vec{v}_1 \vec{S}_1 \cdot \vec{v}_1 \hat{n} \cdot \vec{S}_1 - \frac{13}{2} \hat{n} \cdot \vec{v}_2 \vec{S}_1 \cdot \vec{v}_1 \hat{n} \cdot \vec{S}_1 - \frac{13}{2} \hat{n} \cdot \vec{v}_1 \vec{S}_1 \cdot \vec{v}_2 \hat{n} \cdot \vec{S}_1 + \right. \\ \left. \frac{11}{2} \hat{n} \cdot \vec{v}_2 \vec{S}_1 \cdot \vec{v}_2 \hat{n} \cdot \vec{S}_1 - \frac{1}{2} (\vec{S}_1 \cdot \vec{v}_1)^2 - \frac{49}{100} (\vec{S}_1 \cdot \vec{v}_2)^2 - \frac{5}{2} (\hat{n} \cdot \vec{v}_1)^2 \vec{S}_1 \cdot \vec{S}_1 + \frac{17}{8} (\hat{n} \cdot \vec{v}_2)^2 \vec{S}_1 \cdot \vec{S}_1 - \right. \\ \left. 7 \hat{n} \cdot \vec{v}_1 \hat{n} \cdot \vec{v}_2 \vec{S}_1 \cdot \vec{S}_1 + \vec{S}_1 \cdot \vec{v}_1 \vec{S}_1 \cdot \vec{v}_2 + \frac{11}{4} \vec{S}_1 \cdot \vec{S}_1 \vec{v}_1 \cdot \vec{v}_1 + \frac{5}{4} \vec{S}_1 \cdot \vec{S}_1 \vec{v}_1 \cdot \vec{v}_2 + \frac{1151}{200} \vec{S}_1 \cdot \vec{S}_1 \vec{v}_2 \cdot \vec{v}_2 \right) + \right. \\ \left. \left( \frac{\frac{15}{2} \hat{n} \cdot \vec{S}_1 \hat{n} \cdot \vec{S}_1 \hat{n} \cdot \vec{v}_2 - \frac{3}{2} \vec{S}_1 \cdot \vec{S}_1 \hat{n} \cdot \vec{v}_2 - \frac{3}{2} \hat{n} \cdot \vec{S}_1 \vec{S}_1 \cdot \vec{v}_2 - \frac{3}{2} \hat{n} \cdot \vec{S}_1 \vec{S}_1 \cdot \vec{v}_2}{r^4} + \frac{1}{r^5} \right. \right. \\ \left( \frac{21}{4} (\hat{n} \cdot \vec{v}_2)^2 (\hat{n} \cdot \vec{S}_1)^2 - \frac{105}{4} \hat{n} \cdot \vec{v}_1 \hat{n} \cdot \vec{v}_2 (\hat{n} \cdot \vec{S}_1)^2 + \frac{15}{4} \vec{v}_1 \cdot \vec{v}_2 (\hat{n} \cdot \vec{S}_1)^2 - \frac{3}{4} \vec{v}_2 \cdot \vec{v}_2 (\hat{n} \cdot \vec{S}_1)^2 + \right. \\ \left. \frac{15}{2} \hat{n} \cdot \vec{v}_2 \vec{S}_1 \cdot \vec{v}_1 \hat{n} \cdot \vec{S}_1 + \frac{15}{2} \hat{n} \cdot \vec{v}_1 \vec{S}_1 \cdot \vec{v}_2 \hat{n} \cdot \vec{S}_1 - 3 \hat{n} \cdot \vec{v}_2 \vec{S}_1 \cdot \vec{v}_2 \hat{n} \cdot \vec{S}_1 + \frac{3}{10} (\vec{S}_1 \cdot \vec{v}_2)^2 - \frac{3}{4} (\hat{n} \cdot \vec{v}_2)^2 \vec{S}_1 \cdot \vec{S}_1 + \right. \\ \left. \frac{15}{4} \hat{n} \cdot \vec{v}_1 \hat{n} \cdot \vec{v}_2 \vec{S}_1 \cdot \vec{S}_1 - \frac{3}{2} \vec{S}_1 \cdot \vec{v}_1 \vec{S}_1 \cdot \vec{v}_2 - \frac{3}{4} \vec{S}_1 \cdot \vec{S}_1 \vec{v}_1 \cdot \vec{v}_2 + \frac{3}{20} \vec{S}_1 \cdot \vec{S}_1 \vec{v}_2 \cdot \vec{v}_2 \right) \Bigg) \log \left( \frac{r}{R_\theta} \right) + \right. \\ \left. \frac{\vec{S}_1^2}{3r^3} + \frac{1}{\epsilon_d} \left( \frac{-\frac{5}{2} \hat{n} \cdot \vec{S}_1 \hat{n} \cdot \vec{S}_1 \hat{n} \cdot \vec{v}_2 + \frac{1}{2} \vec{S}_1 \cdot \vec{S}_1 \hat{n} \cdot \vec{v}_2 + \frac{1}{2} \hat{n} \cdot \vec{S}_1 \vec{S}_1 \cdot \vec{v}_2 + \frac{1}{2} \hat{n} \cdot \vec{S}_1 \vec{S}_1 \cdot \vec{v}_2}{r^4} + \frac{1}{r^5} \right. \right. \\ \left( -\frac{7}{4} (\hat{n} \cdot \vec{v}_2)^2 (\hat{n} \cdot \vec{S}_1)^2 + \frac{35}{4} \hat{n} \cdot \vec{v}_1 \hat{n} \cdot \vec{v}_2 (\hat{n} \cdot \vec{S}_1)^2 - \frac{5}{4} \vec{v}_1 \cdot \vec{v}_2 (\hat{n} \cdot \vec{S}_1)^2 + \frac{1}{4} \vec{v}_2 \cdot \vec{v}_2 (\hat{n} \cdot \vec{S}_1)^2 - \right. \\ \left. \frac{5}{2} \hat{n} \cdot \vec{v}_2 \vec{S}_1 \cdot \vec{v}_1 \hat{n} \cdot \vec{S}_1 - \frac{5}{2} \hat{n} \cdot \vec{v}_1 \vec{S}_1 \cdot \vec{v}_2 \hat{n} \cdot \vec{S}_1 + \hat{n} \cdot \vec{v}_2 \vec{S}_1 \cdot \vec{v}_2 \hat{n} \cdot \vec{S}_1 - \frac{1}{10} (\vec{S}_1 \cdot \vec{v}_2)^2 + \frac{1}{4} (\hat{n} \cdot \vec{v}_2)^2 \vec{S}_1 \cdot \vec{S}_1 - \right. \\ \left. \frac{5}{4} \hat{n} \cdot \vec{v}_1 \hat{n} \cdot \vec{v}_2 \vec{S}_1 \cdot \vec{S}_1 + \frac{1}{2} \vec{S}_1 \cdot \vec{v}_1 \vec{S}_1 \cdot \vec{v}_2 + \frac{1}{4} \vec{S}_1 \cdot \vec{S}_1 \vec{v}_1 \cdot \vec{v}_2 - \frac{1}{20} \vec{S}_1 \cdot \vec{S}_1 \vec{v}_2 \cdot \vec{v}_2 \right) \Bigg) \Bigg\} c_{\text{ES}^2 1}$$

$\{\text{DiagS1CES2}[3, 1, 51],$

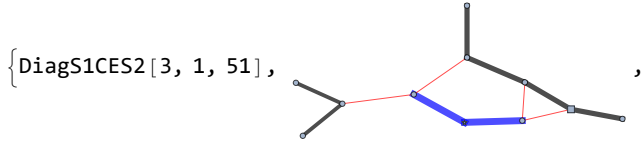

,

$$\begin{aligned}
 & G^3 m_1 m_2 \left( \frac{1}{r^4} \left( -\frac{68}{147} \hat{n} \cdot \vec{S}_1 \hat{n} \cdot \vec{S}_1 \hat{n} \cdot \vec{v}_1 + \frac{277 \vec{S}_1 \cdot \vec{S}_1 \hat{n} \cdot \vec{v}_1}{3675} - \frac{1}{2} \hat{n} \cdot \vec{S}_1 \hat{n} \cdot \vec{S}_1 \hat{n} \cdot \vec{v}_2 + \right. \right. \\
 & \quad \left. \frac{1079 \hat{n} \cdot \vec{S}_1 \vec{S}_1 \cdot \vec{v}_1}{7350} + \frac{1}{10} \hat{n} \cdot \vec{S}_1 \vec{S}_1 \cdot \vec{v}_2 + \frac{1}{10} \hat{n} \cdot \vec{v}_2 \vec{S}_1 \cdot \vec{S}_1 + \frac{1079 \hat{n} \cdot \vec{S}_1 \vec{S}_1 \cdot \vec{v}_1}{7350} + \frac{1}{10} \hat{n} \cdot \vec{S}_1 \vec{S}_1 \cdot \vec{v}_2 \right) + \\
 & \quad \frac{1}{r^5} \left( \frac{3}{16} (\hat{n} \cdot \vec{v}_1)^2 (\hat{n} \cdot \vec{S}_1)^2 + \frac{43}{12} \hat{n} \cdot \vec{v}_1 \hat{n} \cdot \vec{v}_2 (\hat{n} \cdot \vec{S}_1)^2 - \frac{107 \vec{v}_1 \cdot \vec{v}_1 (\hat{n} \cdot \vec{S}_1)^2}{2352} - \frac{283}{588} \vec{v}_1 \cdot \vec{v}_2 (\hat{n} \cdot \vec{S}_1)^2 - \right. \\
 & \quad \frac{149}{588} \hat{n} \cdot \vec{v}_1 \vec{S}_1 \cdot \vec{v}_1 \hat{n} \cdot \vec{S}_1 - \frac{194}{147} \hat{n} \cdot \vec{v}_2 \vec{S}_1 \cdot \vec{v}_1 \hat{n} \cdot \vec{S}_1 - \frac{283}{294} \hat{n} \cdot \vec{v}_1 \vec{S}_1 \cdot \vec{v}_2 \hat{n} \cdot \vec{S}_1 + \frac{1177 (\vec{S}_1 \cdot \vec{v}_1)^2}{9800} + \\
 & \quad \left. \frac{11}{784} (\hat{n} \cdot \vec{v}_1)^2 \vec{S}_1 \cdot \vec{S}_1 - \frac{283}{588} \hat{n} \cdot \vec{v}_1 \hat{n} \cdot \vec{v}_2 \vec{S}_1 \cdot \vec{S}_1 + \frac{907 \vec{S}_1 \cdot \vec{v}_1 \vec{S}_1 \cdot \vec{v}_2}{3675} - \frac{1369 \vec{S}_1 \cdot \vec{S}_1 \vec{v}_1 \cdot \vec{v}_1}{58800} + \frac{1289 \vec{S}_1 \cdot \vec{S}_1 \vec{v}_1 \cdot \vec{v}_2}{14700} \right) + \\
 & \quad \left( \frac{\frac{3}{7} \hat{n} \cdot \vec{S}_1 \hat{n} \cdot \vec{S}_1 \hat{n} \cdot \vec{v}_1 - \frac{3}{35} \vec{S}_1 \cdot \vec{S}_1 \hat{n} \cdot \vec{v}_1 - \frac{3}{35} \hat{n} \cdot \vec{S}_1 \vec{S}_1 \cdot \vec{v}_1 - \frac{3}{35} \hat{n} \cdot \vec{S}_1 \vec{S}_1 \cdot \vec{v}_1}{r^4} + \frac{1}{r^5} \right. \\
 & \quad \left( -\frac{1}{4} (\hat{n} \cdot \vec{v}_1)^2 (\hat{n} \cdot \vec{S}_1)^2 - \frac{3}{2} \hat{n} \cdot \vec{v}_1 \hat{n} \cdot \vec{v}_2 (\hat{n} \cdot \vec{S}_1)^2 + \frac{1}{28} \vec{v}_1 \cdot \vec{v}_1 (\hat{n} \cdot \vec{S}_1)^2 + \frac{3}{14} \vec{v}_1 \cdot \vec{v}_2 (\hat{n} \cdot \vec{S}_1)^2 + \right. \\
 & \quad \frac{1}{7} \hat{n} \cdot \vec{v}_1 \vec{S}_1 \cdot \vec{v}_1 \hat{n} \cdot \vec{S}_1 + \frac{3}{7} \hat{n} \cdot \vec{v}_2 \vec{S}_1 \cdot \vec{v}_1 \hat{n} \cdot \vec{S}_1 + \frac{3}{7} \hat{n} \cdot \vec{v}_1 \vec{S}_1 \cdot \vec{v}_2 \hat{n} \cdot \vec{S}_1 - \frac{1}{70} (\vec{S}_1 \cdot \vec{v}_1)^2 + \frac{1}{28} (\hat{n} \cdot \vec{v}_1)^2 \vec{S}_1 \cdot \vec{S}_1 + \\
 & \quad \left. \frac{3}{14} \hat{n} \cdot \vec{v}_1 \hat{n} \cdot \vec{v}_2 \vec{S}_1 \cdot \vec{S}_1 - \frac{3}{35} \vec{S}_1 \cdot \vec{v}_1 \vec{S}_1 \cdot \vec{v}_2 - \frac{1}{140} \vec{S}_1 \cdot \vec{S}_1 \vec{v}_1 \cdot \vec{v}_1 - \frac{3}{70} \vec{S}_1 \cdot \vec{S}_1 \vec{v}_1 \cdot \vec{v}_2 \right) \log \left( \frac{r}{R_\theta} \right) + \\
 & \quad \frac{1}{\epsilon_d} \left( \frac{-\frac{1}{7} \hat{n} \cdot \vec{S}_1 \hat{n} \cdot \vec{S}_1 \hat{n} \cdot \vec{v}_1 + \frac{1}{35} \vec{S}_1 \cdot \vec{S}_1 \hat{n} \cdot \vec{v}_1 + \frac{1}{35} \hat{n} \cdot \vec{S}_1 \vec{S}_1 \cdot \vec{v}_1 + \frac{1}{35} \hat{n} \cdot \vec{S}_1 \vec{S}_1 \cdot \vec{v}_1}{r^4} + \frac{1}{r^5} \right. \\
 & \quad \left( \frac{1}{12} (\hat{n} \cdot \vec{v}_1)^2 (\hat{n} \cdot \vec{S}_1)^2 + \frac{1}{2} \hat{n} \cdot \vec{v}_1 \hat{n} \cdot \vec{v}_2 (\hat{n} \cdot \vec{S}_1)^2 - \frac{1}{84} \vec{v}_1 \cdot \vec{v}_1 (\hat{n} \cdot \vec{S}_1)^2 - \frac{1}{14} \vec{v}_1 \cdot \vec{v}_2 (\hat{n} \cdot \vec{S}_1)^2 - \right. \\
 & \quad \frac{1}{21} \hat{n} \cdot \vec{v}_1 \vec{S}_1 \cdot \vec{v}_1 \hat{n} \cdot \vec{S}_1 - \frac{1}{7} \hat{n} \cdot \vec{v}_2 \vec{S}_1 \cdot \vec{v}_1 \hat{n} \cdot \vec{S}_1 - \frac{1}{7} \hat{n} \cdot \vec{v}_1 \vec{S}_1 \cdot \vec{v}_2 \hat{n} \cdot \vec{S}_1 + \frac{1}{210} (\vec{S}_1 \cdot \vec{v}_1)^2 - \frac{1}{84} (\hat{n} \cdot \vec{v}_1)^2 \vec{S}_1 \cdot \vec{S}_1 - \\
 & \quad \left. \frac{1}{14} \hat{n} \cdot \vec{v}_1 \hat{n} \cdot \vec{v}_2 \vec{S}_1 \cdot \vec{S}_1 + \frac{1}{35} \vec{S}_1 \cdot \vec{v}_1 \vec{S}_1 \cdot \vec{v}_2 + \frac{1}{420} \vec{S}_1 \cdot \vec{S}_1 \vec{v}_1 \cdot \vec{v}_1 + \frac{1}{70} \vec{S}_1 \cdot \vec{S}_1 \vec{v}_1 \cdot \vec{v}_2 \right) \Bigg) \Bigg\} C_{\text{ES}^2 1}
 \end{aligned}$$

$\{\text{DiagS1CES2}[3, 1, 52],$

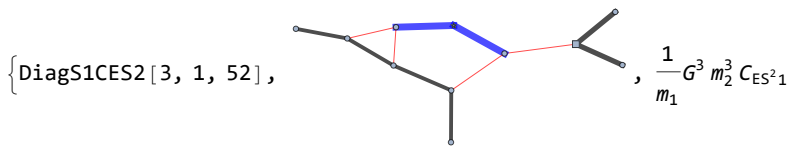

,  $\frac{1}{m_1} G^3 m_2^3 C_{\text{ES}^2 1}$

$$\begin{aligned}
& \left( \frac{\frac{7}{4} (\hat{n} \cdot \vec{S}_1)^2 (\hat{n} \cdot \vec{v}_2)^2 - \frac{1}{4} \vec{v}_2 \cdot \vec{v}_2 (\hat{n} \cdot \vec{S}_1)^2 - \hat{n} \cdot \vec{S}_1 \hat{n} \cdot \vec{v}_2 \vec{S}_1 \cdot \vec{v}_2 - \frac{1}{4} \vec{S}_1 \cdot \vec{S}_1 (\hat{n} \cdot \vec{v}_2)^2 + \frac{1}{10} (\vec{S}_1 \cdot \vec{v}_2)^2 + \frac{1}{20} \vec{S}_1 \cdot \vec{S}_1 \vec{v}_2 \cdot \vec{v}_2}{r^5 \in_d} + \right. \\
& \frac{1}{r^5} \log \left( \frac{r}{R_\theta} \right) \left( -\frac{21}{4} (\hat{n} \cdot \vec{S}_1)^2 (\hat{n} \cdot \vec{v}_2)^2 + \frac{3}{4} \vec{v}_2 \cdot \vec{v}_2 (\hat{n} \cdot \vec{S}_1)^2 + \right. \\
& \quad \left. 3 \hat{n} \cdot \vec{S}_1 \hat{n} \cdot \vec{v}_2 \vec{S}_1 \cdot \vec{v}_2 + \frac{3}{4} \vec{S}_1 \cdot \vec{S}_1 (\hat{n} \cdot \vec{v}_2)^2 - \frac{3}{10} (\vec{S}_1 \cdot \vec{v}_2)^2 - \frac{3}{20} \vec{S}_1 \cdot \vec{S}_1 \vec{v}_2 \cdot \vec{v}_2 \right) + \frac{1}{r^5} \\
& \left( \frac{109}{24} (\hat{n} \cdot \vec{S}_1)^2 (\hat{n} \cdot \vec{v}_2)^2 + \frac{35}{6} (\hat{n} \cdot \vec{S}_1)^2 \hat{n} \cdot \vec{v}_1 \hat{n} \cdot \vec{v}_2 - \frac{5}{6} \vec{v}_1 \cdot \vec{v}_2 (\hat{n} \cdot \vec{S}_1)^2 - \frac{37}{24} \vec{v}_2 \cdot \vec{v}_2 (\hat{n} \cdot \vec{S}_1)^2 - \right. \\
& \quad \frac{5}{3} \hat{n} \cdot \vec{S}_1 \hat{n} \cdot \vec{v}_2 \vec{S}_1 \cdot \vec{v}_1 - \frac{5}{3} \hat{n} \cdot \vec{S}_1 \hat{n} \cdot \vec{v}_1 \vec{S}_1 \cdot \vec{v}_2 - \frac{13}{6} \hat{n} \cdot \vec{S}_1 \hat{n} \cdot \vec{v}_2 \vec{S}_1 \cdot \vec{v}_2 - \frac{31}{24} \vec{S}_1 \cdot \vec{S}_1 (\hat{n} \cdot \vec{v}_2)^2 - \frac{5}{6} \vec{S}_1 \cdot \vec{S}_1 \hat{n} \cdot \vec{v}_1 \hat{n} \cdot \vec{v}_2 + \\
& \quad \frac{47}{300} (\vec{S}_1 \cdot \vec{v}_2)^2 + \frac{1}{3} \vec{S}_1 \cdot \vec{v}_1 \vec{S}_1 \cdot \vec{v}_2 + \frac{1}{6} \vec{S}_1 \cdot \vec{S}_1 \vec{v}_1 \cdot \vec{v}_2 + \frac{497}{600} \vec{S}_1 \cdot \vec{S}_1 \vec{v}_2 \cdot \vec{v}_2 \Big) + \\
& \quad \left. \left. - \frac{5}{3} \hat{n} \cdot \vec{S}_1 \hat{n} \cdot \vec{S}_1 \hat{n} \cdot \vec{v}_2 + \frac{1}{3} \vec{S}_1 \cdot \vec{S}_1 \hat{n} \cdot \vec{v}_2 + \frac{1}{3} \hat{n} \cdot \vec{S}_1 \vec{S}_1 \cdot \vec{v}_2 + \frac{1}{3} \hat{n} \cdot \vec{S}_1 \vec{S}_1 \cdot \vec{v}_2 \right) \right\} \\
& \quad \left. \frac{1}{r^4} \right\}
\end{aligned}$$

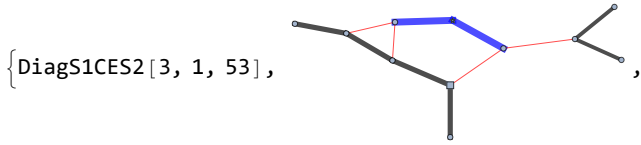

$$\begin{aligned}
& G^3 m_1 m_2 \left( \frac{-\frac{209}{147} \hat{n} \cdot \vec{S}_1 \hat{n} \cdot \vec{S}_1 \hat{n} \cdot \vec{v}_1 + \frac{793 \vec{S}_1 \cdot \vec{S}_1 \hat{n} \cdot \vec{v}_1}{3675} + \frac{1843 \hat{n} \cdot \vec{S}_1 \vec{S}_1 \cdot \vec{v}_1}{3675} + \frac{1843 \hat{n} \cdot \vec{S}_1 \vec{S}_1 \cdot \vec{v}_1}{3675}}{r^4} + \frac{1}{r^5} \right. \\
& \left( \frac{145}{24} (\hat{n} \cdot \vec{v}_1)^2 (\hat{n} \cdot \vec{S}_1)^2 - \frac{35}{6} \hat{n} \cdot \vec{v}_1 \hat{n} \cdot \vec{v}_2 (\hat{n} \cdot \vec{S}_1)^2 - \frac{1565 \vec{v}_1 \cdot \vec{v}_1 (\hat{n} \cdot \vec{S}_1)^2}{1176} + \frac{209}{294} \vec{v}_1 \cdot \vec{v}_2 (\hat{n} \cdot \vec{S}_1)^2 - \right. \\
& \quad \frac{1145}{294} \hat{n} \cdot \vec{v}_1 \vec{S}_1 \cdot \vec{v}_1 \hat{n} \cdot \vec{S}_1 + \frac{419}{147} \hat{n} \cdot \vec{v}_2 \vec{S}_1 \cdot \vec{v}_1 \hat{n} \cdot \vec{S}_1 + \frac{209}{147} \hat{n} \cdot \vec{v}_1 \vec{S}_1 \cdot \vec{v}_2 \hat{n} \cdot \vec{S}_1 + \frac{299}{588} (\vec{S}_1 \cdot \vec{v}_1)^2 - \\
& \quad \left. \frac{1075 (\hat{n} \cdot \vec{v}_1)^2 \vec{S}_1 \cdot \vec{S}_1}{1176} + \frac{209}{294} \hat{n} \cdot \vec{v}_1 \hat{n} \cdot \vec{v}_2 \vec{S}_1 \cdot \vec{S}_1 - \frac{1843 \vec{S}_1 \cdot \vec{v}_1 \vec{S}_1 \cdot \vec{v}_2}{3675} + \frac{123}{392} \vec{S}_1 \cdot \vec{S}_1 \vec{v}_1 \cdot \vec{v}_1 - \frac{793 \vec{S}_1 \cdot \vec{S}_1 \vec{v}_1 \cdot \vec{v}_2}{7350} \right) + \\
& \left( \frac{\frac{12}{7} \hat{n} \cdot \vec{S}_1 \hat{n} \cdot \vec{S}_1 \hat{n} \cdot \vec{v}_1 - \frac{12}{35} \vec{S}_1 \cdot \vec{S}_1 \hat{n} \cdot \vec{v}_1 - \frac{12}{35} \hat{n} \cdot \vec{S}_1 \vec{S}_1 \cdot \vec{v}_1 - \frac{12}{35} \hat{n} \cdot \vec{S}_1 \vec{S}_1 \cdot \vec{v}_1}{r^4} + \frac{1}{r^5} \right. \\
& \quad \left( -\frac{25}{4} (\hat{n} \cdot \vec{v}_1)^2 (\hat{n} \cdot \vec{S}_1)^2 + 6 \hat{n} \cdot \vec{v}_1 \hat{n} \cdot \vec{v}_2 (\hat{n} \cdot \vec{S}_1)^2 + \frac{25}{28} \vec{v}_1 \cdot \vec{v}_1 (\hat{n} \cdot \vec{S}_1)^2 - \frac{6}{7} \vec{v}_1 \cdot \vec{v}_2 (\hat{n} \cdot \vec{S}_1)^2 + \right. \\
& \quad \frac{25}{7} \hat{n} \cdot \vec{v}_1 \vec{S}_1 \cdot \vec{v}_1 \hat{n} \cdot \vec{S}_1 - \frac{12}{7} \hat{n} \cdot \vec{v}_2 \vec{S}_1 \cdot \vec{v}_1 \hat{n} \cdot \vec{S}_1 - \frac{12}{7} \hat{n} \cdot \vec{v}_1 \vec{S}_1 \cdot \vec{v}_2 \hat{n} \cdot \vec{S}_1 - \frac{5}{14} (\vec{S}_1 \cdot \vec{v}_1)^2 + \frac{25}{28} (\hat{n} \cdot \vec{v}_1)^2 \vec{S}_1 \cdot \vec{S}_1 - \\
& \quad \left. \frac{6}{7} \hat{n} \cdot \vec{v}_1 \hat{n} \cdot \vec{v}_2 \vec{S}_1 \cdot \vec{S}_1 + \frac{12}{35} \vec{S}_1 \cdot \vec{v}_1 \vec{S}_1 \cdot \vec{v}_2 - \frac{5}{28} \vec{S}_1 \cdot \vec{S}_1 \vec{v}_1 \cdot \vec{v}_1 + \frac{6}{35} \vec{S}_1 \cdot \vec{S}_1 \vec{v}_1 \cdot \vec{v}_2 \right) \log \left( \frac{r}{R_\theta} \right) + \\
& \quad \left. \frac{1}{\epsilon_d} \left( \frac{-\frac{4}{7} \hat{n} \cdot \vec{S}_1 \hat{n} \cdot \vec{S}_1 \hat{n} \cdot \vec{v}_1 + \frac{4}{35} \vec{S}_1 \cdot \vec{S}_1 \hat{n} \cdot \vec{v}_1 + \frac{4}{35} \hat{n} \cdot \vec{S}_1 \vec{S}_1 \cdot \vec{v}_1 + \frac{4}{35} \hat{n} \cdot \vec{S}_1 \vec{S}_1 \cdot \vec{v}_1}{r^4} + \frac{1}{r^5} \right. \right. \\
& \quad \left. \left( \frac{25}{12} (\hat{n} \cdot \vec{v}_1)^2 (\hat{n} \cdot \vec{S}_1)^2 - 2 \hat{n} \cdot \vec{v}_1 \hat{n} \cdot \vec{v}_2 (\hat{n} \cdot \vec{S}_1)^2 - \frac{25}{84} \vec{v}_1 \cdot \vec{v}_1 (\hat{n} \cdot \vec{S}_1)^2 + \frac{2}{7} \vec{v}_1 \cdot \vec{v}_2 (\hat{n} \cdot \vec{S}_1)^2 - \right. \right.
\end{aligned}$$

$$\frac{25}{21} \hat{n} \cdot \vec{v}_1 \vec{S}_1 \cdot \vec{v}_1 \hat{n} \cdot \vec{S}_1 + \frac{4}{7} \hat{n} \cdot \vec{v}_2 \vec{S}_1 \cdot \vec{v}_1 \hat{n} \cdot \vec{S}_1 + \frac{4}{7} \hat{n} \cdot \vec{v}_1 \vec{S}_1 \cdot \vec{v}_2 \hat{n} \cdot \vec{S}_1 + \frac{5}{42} (\vec{S}_1 \cdot \vec{v}_1)^2 - \frac{25}{84} (\hat{n} \cdot \vec{v}_1)^2 \vec{S}_1 \cdot \vec{S}_1 +$$

$$\frac{2}{7} \hat{n} \cdot \vec{v}_1 \hat{n} \cdot \vec{v}_2 \vec{S}_1 \cdot \vec{S}_1 - \frac{4}{35} \vec{S}_1 \cdot \vec{v}_1 \vec{S}_1 \cdot \vec{v}_2 + \frac{5}{84} \vec{S}_1 \cdot \vec{S}_1 \vec{v}_1 \cdot \vec{v}_1 - \frac{2}{35} \vec{S}_1 \cdot \vec{S}_1 \vec{v}_1 \cdot \vec{v}_2 \Bigg) \Bigg\} C_{ES^2_1}$$

{DiagS1CES2[3, 2, 1],

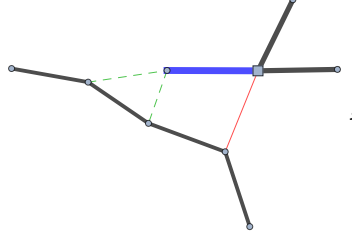

$$\frac{G^3 m_2^3 C_{ES^2_1} \left( -18 \vec{v}_2 \cdot \vec{v}_2 (\hat{n} \cdot \vec{S}_1)^2 + 20 \hat{n} \cdot \vec{S}_1 \hat{n} \cdot \vec{v}_2 \vec{S}_1 \cdot \vec{v}_2 - 20 \vec{S}_1 \cdot \vec{S}_1 (\hat{n} \cdot \vec{v}_2)^2 - 8 (\vec{S}_1 \cdot \vec{v}_2)^2 + 14 \vec{S}_1 \cdot \vec{S}_1 \vec{v}_2 \cdot \vec{v}_2 \right)}{m_1 r^5}$$

{DiagS1CES2[3, 2, 2],

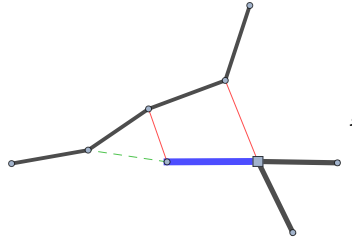

$$\frac{G^3 m_2^3 C_{ES^2_1} \left( -20 \hat{n} \cdot \vec{a}_2 (\hat{n} \cdot \vec{S}_1)^2 - 4 \vec{S}_1 \cdot \vec{a}_2 \hat{n} \cdot \vec{S}_1 + 16 \vec{S}_1 \cdot \vec{S}_1 \hat{n} \cdot \vec{a}_2 \right)}{m_1 r^4}$$

{DiagS1CES2[3, 2, 3],

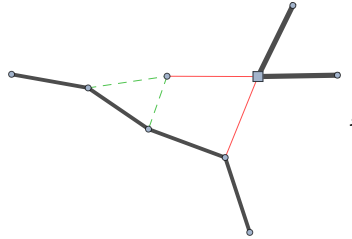

$$\frac{G^3 m_2^3 C_{ES^2_1} \left( 90 \vec{v}_2 \cdot \vec{v}_2 (\hat{n} \cdot \vec{S}_1)^2 - 38 \vec{S}_1 \cdot \vec{S}_1 \vec{v}_2 \cdot \vec{v}_2 \right)}{m_1 r^5}$$

{DiagS1CES2[3, 2, 4],

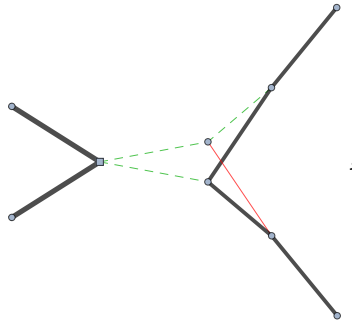

$$\frac{G^3 m_2^3 C_{ES^2_1} \left( 16 \vec{v}_2 \cdot \vec{v}_2 (\hat{n} \cdot \vec{S}_1)^2 - 32 \hat{n} \cdot \vec{S}_1 \hat{n} \cdot \vec{v}_2 \vec{S}_1 \cdot \vec{v}_2 + 32 \vec{S}_1 \cdot \vec{S}_1 (\hat{n} \cdot \vec{v}_2)^2 + 16 (\vec{S}_1 \cdot \vec{v}_2)^2 - 32 \vec{S}_1 \cdot \vec{S}_1 \vec{v}_2 \cdot \vec{v}_2 \right)}{m_1 r^5}$$

$$\left\{ \text{DiagS1CES2}[3, 2, 5], \quad , \quad \frac{1}{m_1} \right.$$

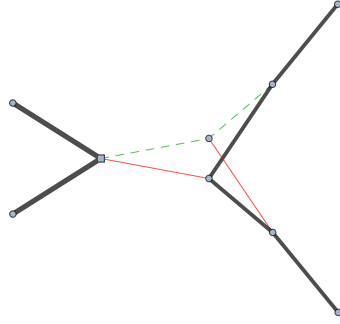

$$G^3 m_2^3 C_{\text{ES}^2 1} \left( \frac{32 \vec{S}_1 \cdot \vec{S}_1 \hat{n} \cdot \vec{a}_2 - 40 \vec{S}_1 \cdot \vec{a}_2 \hat{n} \cdot \vec{S}_1}{r^4} + \frac{1}{r^5} \left( -156 \vec{v}_1 \cdot \vec{v}_2 (\hat{n} \cdot \vec{S}_1)^2 + \right. \right. \\ \left. \left. 8 \hat{n} \cdot \vec{S}_1 \hat{n} \cdot \vec{v}_2 \vec{S}_1 \cdot \vec{v}_1 + 144 \hat{n} \cdot \vec{S}_1 \hat{n} \cdot \vec{v}_1 \vec{S}_1 \cdot \vec{v}_2 - 160 \hat{n} \cdot \vec{S}_1 \hat{n} \cdot \vec{v}_2 \vec{S}_1 \cdot \vec{v}_2 + 144 \vec{S}_1 \cdot \vec{S}_1 (\hat{n} \cdot \vec{v}_2)^2 - \right. \right. \\ \left. \left. 136 \vec{S}_1 \cdot \vec{S}_1 \hat{n} \cdot \vec{v}_1 \hat{n} \cdot \vec{v}_2 + 32 (\vec{S}_1 \cdot \vec{v}_2)^2 - 32 \vec{S}_1 \cdot \vec{v}_1 \vec{S}_1 \cdot \vec{v}_2 + 116 \vec{S}_1 \cdot \vec{S}_1 \vec{v}_1 \cdot \vec{v}_2 - 32 \vec{S}_1 \cdot \vec{S}_1 \vec{v}_2 \cdot \vec{v}_2 \right) \right) \Bigg\}$$

$$\left\{ \text{DiagS1CES2}[3, 2, 6], \quad , \quad \right.$$

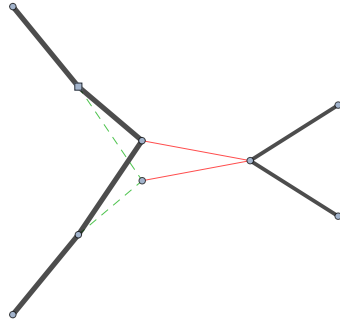

$$G^3 m_1 m_2 C_{\text{ES}^2 1} \left( \frac{12 \vec{v}_1 \cdot \vec{v}_1 (\hat{n} \cdot \vec{S}_1)^2 - 4 \vec{S}_1 \cdot \vec{S}_1 \vec{v}_1 \cdot \vec{v}_1}{r^5} + \frac{-6 \hat{n} \cdot \vec{S}_1 \vec{S}_1 \cdot \vec{v}_1 + 4 \vec{S}_1 \cdot \vec{S}_1 \hat{n} \cdot \vec{v}_1 - 6 \hat{n} \cdot \vec{S}_1 \vec{S}_1 \cdot \vec{v}_1}{r^4} \right) \Bigg\}$$

$$\left\{ \text{DiagS1CES2}[3, 2, 7], \quad , \quad \frac{G^3 m_1 m_2 C_{\text{ES}^2 1} \left( 6 \vec{v}_1 \cdot \vec{v}_1 (\hat{n} \cdot \vec{S}_1)^2 - 2 \vec{S}_1 \cdot \vec{S}_1 \vec{v}_1 \cdot \vec{v}_1 \right)}{r^5} \right\}$$

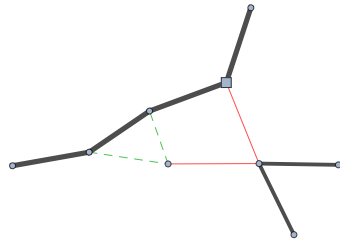

$$\left\{ \text{DiagS1CES2}[3, 2, 8], \quad , \quad \right.$$

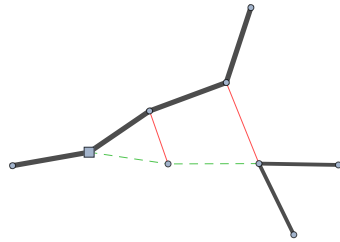

$$G^3 m_1 m_2 C_{\text{ES}^2 1} \left( \frac{-12 \vec{v}_1 \cdot \vec{v}_2 (\hat{n} \cdot \vec{S}_1)^2 + 8 \hat{n} \cdot \vec{S}_1 \hat{n} \cdot \vec{v}_2 \vec{S}_1 \cdot \vec{v}_1 - 8 \hat{n} \cdot \vec{S}_1 \hat{n} \cdot \vec{v}_1 \vec{S}_1 \cdot \vec{v}_2 + 4 \vec{S}_1 \cdot \vec{S}_1 \vec{v}_1 \cdot \vec{v}_2}{r^5} + \right. \\ \left. \frac{6 \hat{n} \cdot \vec{S}_1 \vec{S}_1 \cdot \vec{v}_2 - 4 \vec{S}_1 \cdot \vec{S}_1 \hat{n} \cdot \vec{v}_2 + 6 \hat{n} \cdot \vec{S}_1 \vec{S}_1 \cdot \vec{v}_2}{r^4} \right) \Bigg\}$$



$\{\text{DiagS1CES2}[3, 2, 9],$ 
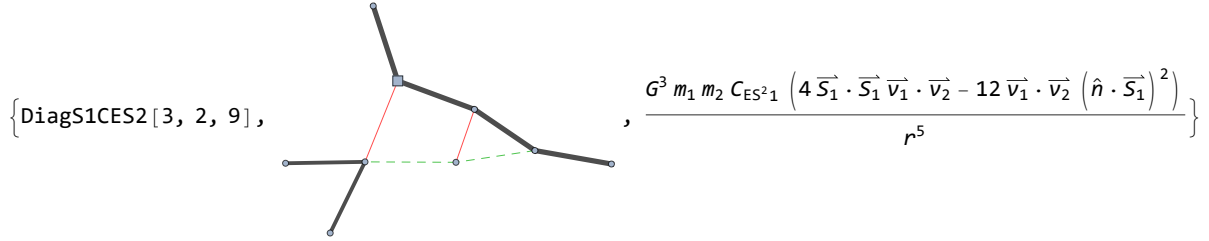
 $, \frac{G^3 m_1 m_2 C_{\text{ES}^2 1} \left( 4 \vec{S}_1 \cdot \vec{S}_1 \vec{v}_1 \cdot \vec{v}_2 - 12 \vec{v}_1 \cdot \vec{v}_2 \left( \hat{n} \cdot \vec{S}_1 \right)^2 \right)}{r^5} \}$

$\{\text{DiagS1CES2}[3, 2, 10],$ 
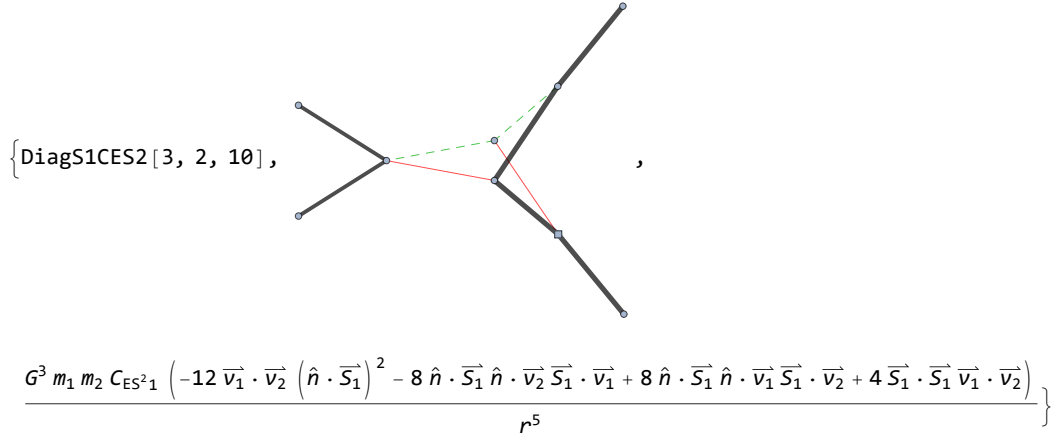
 $, \frac{G^3 m_1 m_2 C_{\text{ES}^2 1} \left( -12 \vec{v}_1 \cdot \vec{v}_2 \left( \hat{n} \cdot \vec{S}_1 \right)^2 - 8 \hat{n} \cdot \vec{S}_1 \hat{n} \cdot \vec{v}_2 \vec{S}_1 \cdot \vec{v}_1 + 8 \hat{n} \cdot \vec{S}_1 \hat{n} \cdot \vec{v}_1 \vec{S}_1 \cdot \vec{v}_2 + 4 \vec{S}_1 \cdot \vec{S}_1 \vec{v}_1 \cdot \vec{v}_2 \right)}{r^5} \}$

$\{\text{DiagS1CES2}[3, 2, 11],$ 
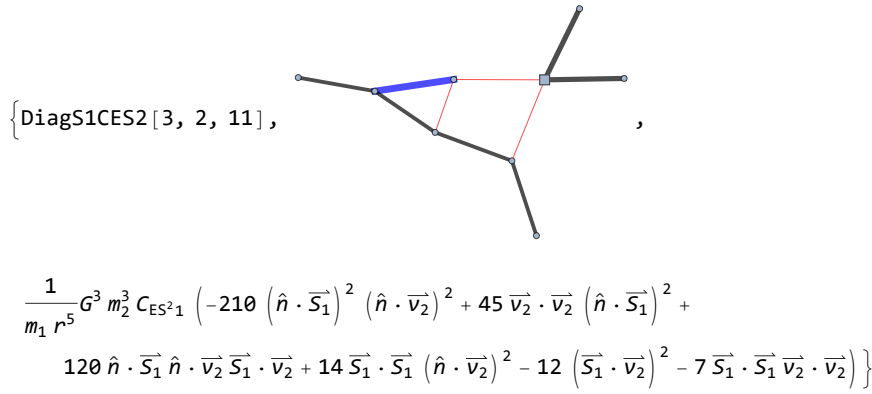
 $, \frac{1}{m_1 r^5} G^3 m_2^3 C_{\text{ES}^2 1} \left( -210 \left( \hat{n} \cdot \vec{S}_1 \right)^2 \left( \hat{n} \cdot \vec{v}_2 \right)^2 + 45 \vec{v}_2 \cdot \vec{v}_2 \left( \hat{n} \cdot \vec{S}_1 \right)^2 + \right.$ 
 $\left. 120 \hat{n} \cdot \vec{S}_1 \hat{n} \cdot \vec{v}_2 \vec{S}_1 \cdot \vec{v}_2 + 14 \vec{S}_1 \cdot \vec{S}_1 \left( \hat{n} \cdot \vec{v}_2 \right)^2 - 12 \left( \vec{S}_1 \cdot \vec{v}_2 \right)^2 - 7 \vec{S}_1 \cdot \vec{S}_1 \vec{v}_2 \cdot \vec{v}_2 \right) \}$

$\{\text{DiagS1CES2}[3, 2, 12],$ 
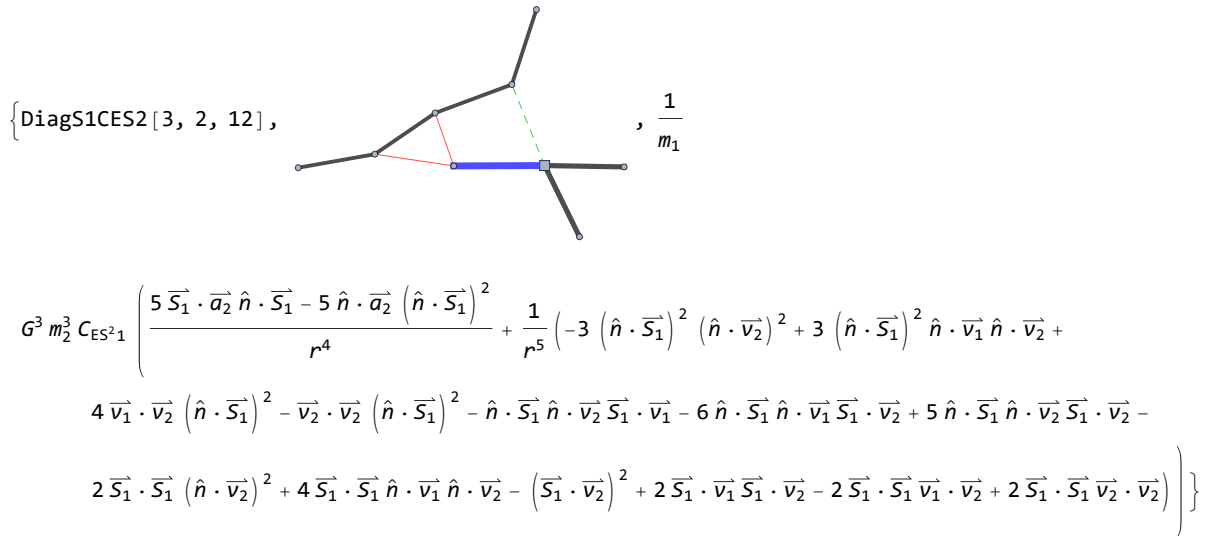
 $, \frac{1}{m_1}$ 
 $G^3 m_2^3 C_{\text{ES}^2 1} \left( \frac{5 \vec{S}_1 \cdot \vec{a}_2 \hat{n} \cdot \vec{S}_1 - 5 \hat{n} \cdot \vec{a}_2 \left( \hat{n} \cdot \vec{S}_1 \right)^2}{r^4} + \frac{1}{r^5} \left( -3 \left( \hat{n} \cdot \vec{S}_1 \right)^2 \left( \hat{n} \cdot \vec{v}_2 \right)^2 + 3 \left( \hat{n} \cdot \vec{S}_1 \right)^2 \hat{n} \cdot \vec{v}_1 \hat{n} \cdot \vec{v}_2 + \right.
 $\left. 4 \vec{v}_1 \cdot \vec{v}_2 \left( \hat{n} \cdot \vec{S}_1 \right)^2 - \vec{v}_2 \cdot \vec{v}_2 \left( \hat{n} \cdot \vec{S}_1 \right)^2 - \hat{n} \cdot \vec{S}_1 \hat{n} \cdot \vec{v}_2 \vec{S}_1 \cdot \vec{v}_1 - 6 \hat{n} \cdot \vec{S}_1 \hat{n} \cdot \vec{v}_1 \vec{S}_1 \cdot \vec{v}_2 + 5 \hat{n} \cdot \vec{S}_1 \hat{n} \cdot \vec{v}_2 \vec{S}_1 \cdot \vec{v}_2 - \right.
 $\left. 2 \vec{S}_1 \cdot \vec{S}_1 \left( \hat{n} \cdot \vec{v}_2 \right)^2 + 4 \vec{S}_1 \cdot \vec{S}_1 \hat{n} \cdot \vec{v}_1 \hat{n} \cdot \vec{v}_2 - \left( \vec{S}_1 \cdot \vec{v}_2 \right)^2 + 2 \vec{S}_1 \cdot \vec{v}_1 \vec{S}_1 \cdot \vec{v}_2 - 2 \vec{S}_1 \cdot \vec{S}_1 \vec{v}_1 \cdot \vec{v}_2 + 2 \vec{S}_1 \cdot \vec{S}_1 \vec{v}_2 \cdot \vec{v}_2 \right) \}$$$

{DiagS1CES2[3, 2, 13],

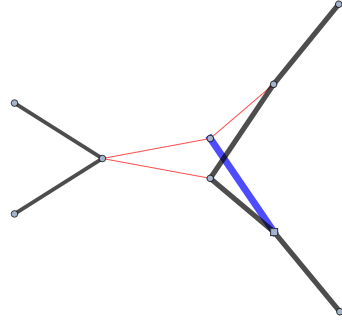

,  $G^3 m_1 m_2 C_{ES^2 1}$

$$\left\{ \frac{2 \hat{n} \cdot \vec{a}_1 \left( \hat{n} \cdot \vec{S}_1 \right)^2 - \vec{S}_1 \cdot \vec{a}_1 \hat{n} \cdot \vec{S}_1 + \vec{S}_1 \cdot \vec{S}_1 \hat{n} \cdot \vec{a}_1 + 8 \hat{n} \cdot \vec{S}_1 \hat{n} \cdot \vec{S}_1 \hat{n} \cdot \vec{v}_1 - \frac{5}{2} \hat{n} \cdot \vec{S}_1 \vec{S}_1 \cdot \vec{v}_1 + 3 \vec{S}_1 \cdot \vec{S}_1 \hat{n} \cdot \vec{v}_1 - \frac{5}{2} \hat{n} \cdot \vec{S}_1 \vec{S}_1 \cdot \vec{v}_1}{r^4} \right. \\ \left. + \frac{-6 \left( \hat{n} \cdot \vec{S}_1 \right)^2 \left( \hat{n} \cdot \vec{v}_1 \right)^2 + \vec{v}_1 \cdot \vec{v}_1 \left( \hat{n} \cdot \vec{S}_1 \right)^2 + 6 \hat{n} \cdot \vec{S}_1 \hat{n} \cdot \vec{v}_1 \vec{S}_1 \cdot \vec{v}_1 - \left( \vec{S}_1 \cdot \vec{v}_1 \right)^2}{r^5} + \frac{-4 \left( \hat{n} \cdot \vec{S}_1 \right)^2 - 4 \hat{n} \cdot \vec{S}_1 \hat{n} \cdot \vec{S}_1}{r^3} \right\}$$

{DiagS1CES2[3, 2, 14],

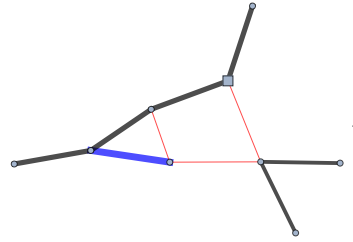

,

$$\frac{G^3 m_1 m_2 C_{ES^2 1} \left( -6 \left( \hat{n} \cdot \vec{S}_1 \right)^2 \left( \hat{n} \cdot \vec{v}_1 \right)^2 + 3 \vec{v}_1 \cdot \vec{v}_1 \left( \hat{n} \cdot \vec{S}_1 \right)^2 + 2 \vec{S}_1 \cdot \vec{S}_1 \left( \hat{n} \cdot \vec{v}_1 \right)^2 - \vec{S}_1 \cdot \vec{S}_1 \vec{v}_1 \cdot \vec{v}_1 \right)}{r^5} \}$$

{DiagS1CES2[3, 2, 15],

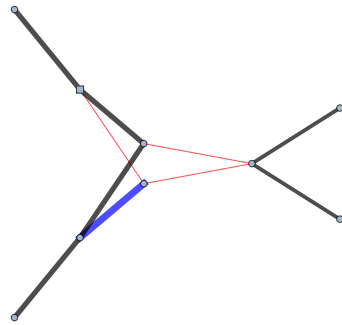

,  $\frac{1}{r^5} G^3 m_1 m_2 C_{ES^2 1}$

$$\left( -30 \left( \hat{n} \cdot \vec{S}_1 \right)^2 \left( \hat{n} \cdot \vec{v}_1 \right)^2 + 5 \vec{v}_1 \cdot \vec{v}_1 \left( \hat{n} \cdot \vec{S}_1 \right)^2 + 18 \hat{n} \cdot \vec{S}_1 \hat{n} \cdot \vec{v}_1 \vec{S}_1 \cdot \vec{v}_1 + 4 \vec{S}_1 \cdot \vec{S}_1 \left( \hat{n} \cdot \vec{v}_1 \right)^2 - 2 \left( \vec{S}_1 \cdot \vec{v}_1 \right)^2 - \vec{S}_1 \cdot \vec{S}_1 \vec{v}_1 \cdot \vec{v}_1 \right) \}$$

{DiagS1CES2[3, 2, 16],

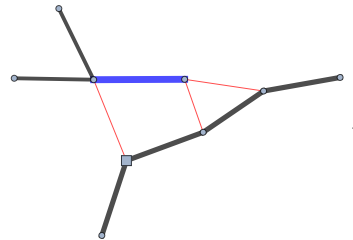

,

$$\frac{G^3 m_1 m_2 C_{ES^2 1} \left( -\frac{9}{4} \left( \hat{n} \cdot \vec{S}_1 \right)^2 \left( \hat{n} \cdot \vec{v}_2 \right)^2 + \frac{9}{4} \vec{v}_2 \cdot \vec{v}_2 \left( \hat{n} \cdot \vec{S}_1 \right)^2 + \frac{3}{4} \vec{S}_1 \cdot \vec{S}_1 \left( \hat{n} \cdot \vec{v}_2 \right)^2 - \frac{3}{4} \vec{S}_1 \cdot \vec{S}_1 \vec{v}_2 \cdot \vec{v}_2 \right)}{r^5} \Bigg\}$$

{DiagS1CES2[3, 2, 17],

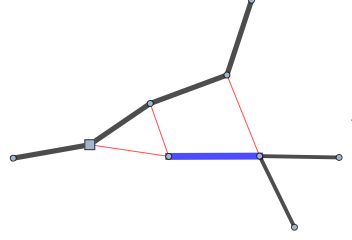

$$\frac{1}{r^5} G^3 m_1 m_2 C_{ES^2 1} \left( -\frac{45}{4} \left( \hat{n} \cdot \vec{S}_1 \right)^2 \left( \hat{n} \cdot \vec{v}_2 \right)^2 + \frac{15}{4} \vec{v}_2 \cdot \vec{v}_2 \left( \hat{n} \cdot \vec{S}_1 \right)^2 + \right. \\ \left. 9 \hat{n} \cdot \vec{S}_1 \hat{n} \cdot \vec{v}_2 \vec{S}_1 \cdot \vec{v}_2 + \frac{3}{4} \vec{S}_1 \cdot \vec{S}_1 \left( \hat{n} \cdot \vec{v}_2 \right)^2 - \frac{3}{2} \left( \vec{S}_1 \cdot \vec{v}_2 \right)^2 - \frac{3}{4} \vec{S}_1 \cdot \vec{S}_1 \vec{v}_2 \cdot \vec{v}_2 \right) \Bigg\}$$

{DiagS1CES2[3, 2, 18],

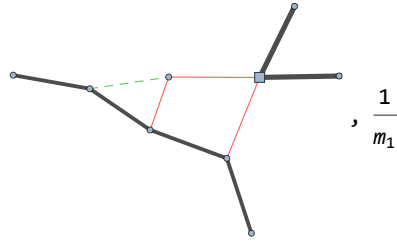

$$G^3 m_2^3 C_{ES^2 1} \left( \frac{1}{r^5} \left( 105 \left( \hat{n} \cdot \vec{S}_1 \right)^2 \left( \hat{n} \cdot \vec{v}_2 \right)^2 + 315 \left( \hat{n} \cdot \vec{S}_1 \right)^2 \hat{n} \cdot \vec{v}_1 \hat{n} \cdot \vec{v}_2 - 45 \vec{v}_1 \cdot \vec{v}_2 \left( \hat{n} \cdot \vec{S}_1 \right)^2 - 45 \vec{v}_2 \cdot \vec{v}_2 \left( \hat{n} \cdot \vec{S}_1 \right)^2 - \right. \right. \\ \left. 90 \hat{n} \cdot \vec{S}_1 \hat{n} \cdot \vec{v}_2 \vec{S}_1 \cdot \vec{v}_1 - 90 \hat{n} \cdot \vec{S}_1 \hat{n} \cdot \vec{v}_1 \vec{S}_1 \cdot \vec{v}_2 - 60 \hat{n} \cdot \vec{S}_1 \hat{n} \cdot \vec{v}_2 \vec{S}_1 \cdot \vec{v}_2 - 3 \vec{S}_1 \cdot \vec{S}_1 \left( \hat{n} \cdot \vec{v}_2 \right)^2 - \right. \\ \left. 25 \vec{S}_1 \cdot \vec{S}_1 \hat{n} \cdot \vec{v}_1 \hat{n} \cdot \vec{v}_2 + 6 \left( \vec{S}_1 \cdot \vec{v}_2 \right)^2 + 18 \vec{S}_1 \cdot \vec{v}_1 \vec{S}_1 \cdot \vec{v}_2 + 5 \vec{S}_1 \cdot \vec{S}_1 \vec{v}_1 \cdot \vec{v}_2 + 9 \vec{S}_1 \cdot \vec{S}_1 \vec{v}_2 \cdot \vec{v}_2 \right) + \\ \left. -90 \hat{n} \cdot \vec{S}_1 \hat{n} \cdot \vec{S}_1 \hat{n} \cdot \vec{v}_2 + 18 \vec{S}_1 \cdot \vec{S}_1 \hat{n} \cdot \vec{v}_2 - 4 \vec{S}_1^2 \hat{n} \cdot \vec{v}_2 + 18 \hat{n} \cdot \vec{S}_1 \vec{S}_1 \cdot \vec{v}_2 + 18 \hat{n} \cdot \vec{S}_1 \vec{S}_1 \cdot \vec{v}_2 \right) \Bigg\}$$

{DiagS1CES2[3, 2, 19],

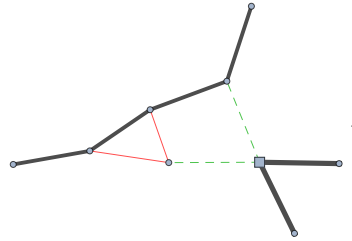

$$\frac{G^3 m_2^3 C_{ES^2 1} \left( - \left( \vec{v}_2 \cdot \vec{v}_2 \right) \left( \hat{n} \cdot \vec{S}_1 \right)^2 + 2 \hat{n} \cdot \vec{S}_1 \hat{n} \cdot \vec{v}_2 \vec{S}_1 \cdot \vec{v}_2 - 2 \vec{S}_1 \cdot \vec{S}_1 \left( \hat{n} \cdot \vec{v}_2 \right)^2 - \left( \vec{S}_1 \cdot \vec{v}_2 \right)^2 + 2 \vec{S}_1 \cdot \vec{S}_1 \vec{v}_2 \cdot \vec{v}_2 \right)}{m_1 r^5} \Bigg\}$$

{DiagS1CES2[3, 2, 20],

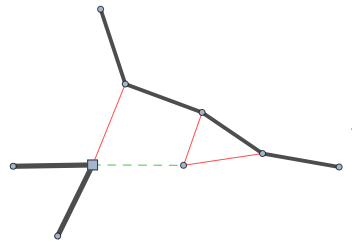

$$\frac{1}{m_1} G^3 m_2^3 C_{ES^2 1} \left( \frac{-8 \hat{n} \cdot \vec{a}_2 \left( \hat{n} \cdot \vec{S}_1 \right)^2 + \frac{13}{2} \vec{S}_1 \cdot \vec{a}_2 \hat{n} \cdot \vec{S}_1 - \frac{3}{2} \vec{S}_1 \cdot \vec{S}_1 \hat{n} \cdot \vec{a}_2}{r^4} + \frac{1}{r^5} \right. \\ \left. \left( -49 \left( \hat{n} \cdot \vec{S}_1 \right)^2 \left( \hat{n} \cdot \vec{v}_2 \right)^2 - \frac{3}{2} \left( \hat{n} \cdot \vec{S}_1 \right)^2 \hat{n} \cdot \vec{v}_1 \hat{n} \cdot \vec{v}_2 + \frac{21}{2} \vec{v}_1 \cdot \vec{v}_2 \left( \hat{n} \cdot \vec{S}_1 \right)^2 + 8 \vec{v}_2 \cdot \vec{v}_2 \left( \hat{n} \cdot \vec{S}_1 \right)^2 - \right. \right. \\ \left. \frac{1}{2} \hat{n} \cdot \vec{S}_1 \hat{n} \cdot \vec{v}_2 \vec{S}_1 \cdot \vec{v}_1 - 9 \hat{n} \cdot \vec{S}_1 \hat{n} \cdot \vec{v}_1 \vec{S}_1 \cdot \vec{v}_2 + \frac{83}{2} \hat{n} \cdot \vec{S}_1 \hat{n} \cdot \vec{v}_2 \vec{S}_1 \cdot \vec{v}_2 - \frac{13}{2} \vec{S}_1 \cdot \vec{S}_1 \left( \hat{n} \cdot \vec{v}_2 \right)^2 + \right. \\ \left. \left. 9 \vec{S}_1 \cdot \vec{S}_1 \hat{n} \cdot \vec{v}_1 \hat{n} \cdot \vec{v}_2 - \frac{11}{2} \left( \vec{S}_1 \cdot \vec{v}_2 \right)^2 + 2 \vec{S}_1 \cdot \vec{v}_1 \vec{S}_1 \cdot \vec{v}_2 - \frac{15}{2} \vec{S}_1 \cdot \vec{S}_1 \vec{v}_1 \cdot \vec{v}_2 + \frac{3}{2} \vec{S}_1 \cdot \vec{S}_1 \vec{v}_2 \cdot \vec{v}_2 \right) \right) \right\}$$

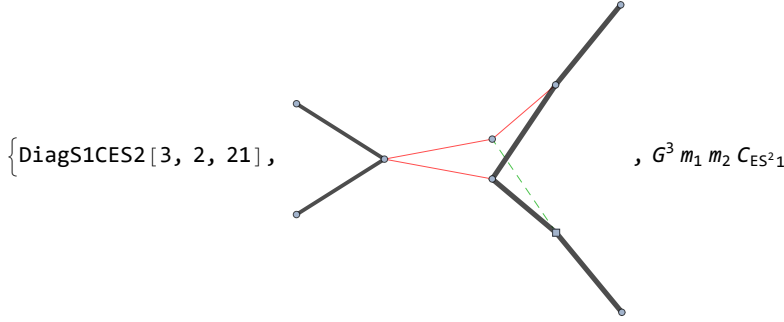

$$\left( \frac{1}{r^5} \left( 5 \left( \hat{n} \cdot \vec{S}_1 \right)^2 \left( \hat{n} \cdot \vec{v}_1 \right)^2 + 7 \left( \hat{n} \cdot \vec{S}_1 \right)^2 \hat{n} \cdot \vec{v}_1 \hat{n} \cdot \vec{v}_2 - \vec{v}_1 \cdot \vec{v}_1 \left( \hat{n} \cdot \vec{S}_1 \right)^2 - \vec{v}_1 \cdot \vec{v}_2 \left( \hat{n} \cdot \vec{S}_1 \right)^2 - 5 \hat{n} \cdot \vec{S}_1 \hat{n} \cdot \vec{v}_1 \vec{S}_1 \cdot \vec{v}_1 - \right. \right. \\ \left. 5 \hat{n} \cdot \vec{S}_1 \hat{n} \cdot \vec{v}_2 \vec{S}_1 \cdot \vec{v}_1 - 2 \hat{n} \cdot \vec{S}_1 \hat{n} \cdot \vec{v}_1 \vec{S}_1 \cdot \vec{v}_2 + \left( \vec{S}_1 \cdot \vec{v}_1 \right)^2 + \vec{S}_1 \cdot \vec{v}_1 \vec{S}_1 \cdot \vec{v}_2 \right) + \frac{1}{r^4} \left( -3 \hat{n} \cdot \vec{S}_1 \hat{n} \cdot \vec{S}_1 \hat{n} \cdot \vec{v}_1 - \right. \\ \left. \left. 5 \hat{n} \cdot \vec{S}_1 \hat{n} \cdot \vec{S}_1 \hat{n} \cdot \vec{v}_2 + \frac{3}{2} \hat{n} \cdot \vec{S}_1 \vec{S}_1 \cdot \vec{v}_1 + \hat{n} \cdot \vec{S}_1 \vec{S}_1 \cdot \vec{v}_2 - 3 \vec{S}_1 \cdot \vec{S}_1 \hat{n} \cdot \vec{v}_2 + \frac{3}{2} \hat{n} \cdot \vec{S}_1 \vec{S}_1 \cdot \vec{v}_1 + \hat{n} \cdot \vec{S}_1 \vec{S}_1 \cdot \vec{v}_2 \right) \right) \right\}$$

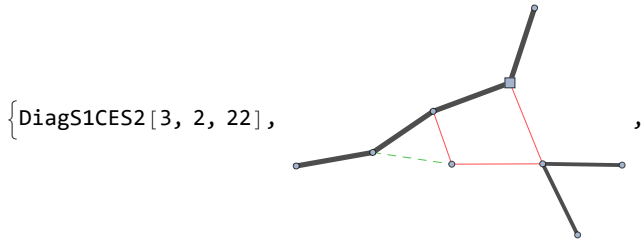

$$G^3 m_1 m_2 C_{ES^2 1} \left( \frac{1}{r^5} \left( -9 \left( \hat{n} \cdot \vec{S}_1 \right)^2 \left( \hat{n} \cdot \vec{v}_1 \right)^2 + 21 \left( \hat{n} \cdot \vec{S}_1 \right)^2 \hat{n} \cdot \vec{v}_1 \hat{n} \cdot \vec{v}_2 - 3 \vec{v}_1 \cdot \vec{v}_1 \left( \hat{n} \cdot \vec{S}_1 \right)^2 - \right. \right. \\ \left. 3 \vec{v}_1 \cdot \vec{v}_2 \left( \hat{n} \cdot \vec{S}_1 \right)^2 + 6 \hat{n} \cdot \vec{S}_1 \hat{n} \cdot \vec{v}_1 \vec{S}_1 \cdot \vec{v}_1 - 6 \hat{n} \cdot \vec{S}_1 \hat{n} \cdot \vec{v}_1 \vec{S}_1 \cdot \vec{v}_2 + \vec{S}_1 \cdot \vec{S}_1 \left( \hat{n} \cdot \vec{v}_1 \right)^2 - \right. \\ \left. \left. 5 \vec{S}_1 \cdot \vec{S}_1 \hat{n} \cdot \vec{v}_1 \hat{n} \cdot \vec{v}_2 + \vec{S}_1 \cdot \vec{S}_1 \vec{v}_1 \cdot \vec{v}_1 + \vec{S}_1 \cdot \vec{S}_1 \vec{v}_1 \cdot \vec{v}_2 \right) + \frac{6 \hat{n} \cdot \vec{S}_1 \hat{n} \cdot \vec{S}_1 \hat{n} \cdot \vec{v}_1 - 2 \vec{S}_1 \cdot \vec{S}_1 \hat{n} \cdot \vec{v}_1}{r^4} \right) \right\}$$

{DiagS1CES2[3, 2, 23],

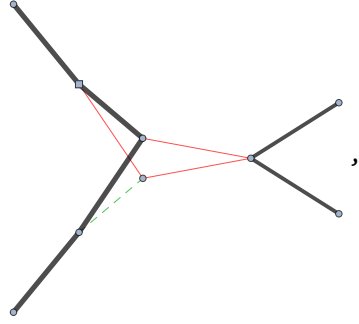

$$G^3 m_1 m_2 C_{ES^2 1} \left\{ \frac{1}{r^5} \left( 25 \left( \hat{n} \cdot \vec{S}_1 \right)^2 \left( \hat{n} \cdot \vec{v}_1 \right)^2 + 35 \left( \hat{n} \cdot \vec{S}_1 \right)^2 \hat{n} \cdot \vec{v}_1 \hat{n} \cdot \vec{v}_2 - 5 \vec{v}_1 \cdot \vec{v}_1 \left( \hat{n} \cdot \vec{S}_1 \right)^2 - 5 \vec{v}_1 \cdot \vec{v}_2 \left( \hat{n} \cdot \vec{S}_1 \right)^2 - \right. \right. \\ \left. \left. 16 \hat{n} \cdot \vec{S}_1 \hat{n} \cdot \vec{v}_1 \vec{S}_1 \cdot \vec{v}_1 - 10 \hat{n} \cdot \vec{S}_1 \hat{n} \cdot \vec{v}_2 \vec{S}_1 \cdot \vec{v}_1 - 10 \hat{n} \cdot \vec{S}_1 \hat{n} \cdot \vec{v}_1 \vec{S}_1 \cdot \vec{v}_2 - 3 \vec{S}_1 \cdot \vec{S}_1 \left( \hat{n} \cdot \vec{v}_1 \right)^2 - \right. \right. \\ \left. \left. 5 \vec{S}_1 \cdot \vec{S}_1 \hat{n} \cdot \vec{v}_1 \hat{n} \cdot \vec{v}_2 + 2 \left( \vec{S}_1 \cdot \vec{v}_1 \right)^2 + 2 \vec{S}_1 \cdot \vec{v}_1 \vec{S}_1 \cdot \vec{v}_2 + \vec{S}_1 \cdot \vec{S}_1 \vec{v}_1 \cdot \vec{v}_1 + \vec{S}_1 \cdot \vec{S}_1 \vec{v}_1 \cdot \vec{v}_2 \right) + \right. \\ \left. \frac{-12 \hat{n} \cdot \vec{S}_1 \hat{n} \cdot \vec{S}_1 \hat{n} \cdot \vec{v}_1 + 2 \vec{S}_1 \cdot \vec{S}_1 \hat{n} \cdot \vec{v}_1 + 3 \hat{n} \cdot \vec{S}_1 \vec{S}_1 \cdot \vec{v}_1 + 3 \hat{n} \cdot \vec{S}_1 \vec{S}_1 \cdot \vec{v}_1}{r^4} \right\}$$

{DiagS1CES2[3, 2, 24],

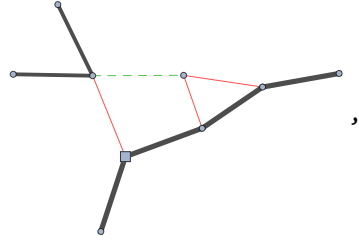

$$G^3 m_1 m_2 C_{ES^2 1} \left\{ \frac{-\frac{3}{2} \left( \hat{n} \cdot \vec{S}_1 \right)^2 \hat{n} \cdot \vec{v}_1 \hat{n} \cdot \vec{v}_2 + \frac{3}{2} \vec{v}_1 \cdot \vec{v}_2 \left( \hat{n} \cdot \vec{S}_1 \right)^2 + \frac{1}{2} \vec{S}_1 \cdot \vec{S}_1 \hat{n} \cdot \vec{v}_1 \hat{n} \cdot \vec{v}_2 - \frac{1}{2} \vec{S}_1 \cdot \vec{S}_1 \vec{v}_1 \cdot \vec{v}_2}{r^5} \right\}$$

{DiagS1CES2[3, 2, 25],

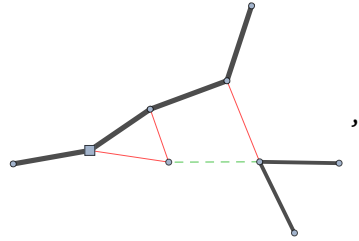

$$G^3 m_1 m_2 C_{ES^2 1} \left\{ \frac{1}{r^5} \left( -\frac{15}{2} \left( \hat{n} \cdot \vec{S}_1 \right)^2 \hat{n} \cdot \vec{v}_1 \hat{n} \cdot \vec{v}_2 + \frac{5}{2} \vec{v}_1 \cdot \vec{v}_2 \left( \hat{n} \cdot \vec{S}_1 \right)^2 + 3 \hat{n} \cdot \vec{S}_1 \hat{n} \cdot \vec{v}_2 \vec{S}_1 \cdot \vec{v}_1 + 3 \hat{n} \cdot \vec{S}_1 \hat{n} \cdot \vec{v}_1 \vec{S}_1 \cdot \vec{v}_2 + \right. \right. \\ \left. \left. \frac{1}{2} \vec{S}_1 \cdot \vec{S}_1 \hat{n} \cdot \vec{v}_1 \hat{n} \cdot \vec{v}_2 - \vec{S}_1 \cdot \vec{v}_1 \vec{S}_1 \cdot \vec{v}_2 - \frac{1}{2} \vec{S}_1 \cdot \vec{S}_1 \vec{v}_1 \cdot \vec{v}_2 \right) + \frac{2 \hat{n} \cdot \vec{S}_1 \hat{n} \cdot \vec{S}_1 \hat{n} \cdot \vec{v}_2 - \hat{n} \cdot \vec{S}_1 \vec{S}_1 \cdot \vec{v}_2 - \hat{n} \cdot \vec{S}_1 \vec{S}_1 \cdot \vec{v}_2}{r^4} \right\}$$

{DiagS1CES2[3, 2, 26],

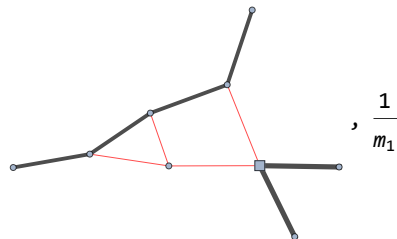

,  $\frac{1}{m_1}$

$$G^3 m_2^3 C_{ES^2 1} \left\{ \frac{1}{r^5} \left( \frac{525}{4} (\hat{n} \cdot \vec{S}_1)^2 (\hat{n} \cdot \vec{v}_2)^2 - 315 (\hat{n} \cdot \vec{S}_1)^2 \hat{n} \cdot \vec{v}_1 \hat{n} \cdot \vec{v}_2 + 45 \vec{v}_1 \cdot \vec{v}_2 (\hat{n} \cdot \vec{S}_1)^2 - \frac{45}{4} \vec{v}_2 \cdot \vec{v}_2 (\hat{n} \cdot \vec{S}_1)^2 + \right. \right. \\
90 \hat{n} \cdot \vec{S}_1 \hat{n} \cdot \vec{v}_2 \vec{S}_1 \cdot \vec{v}_1 + 90 \hat{n} \cdot \vec{S}_1 \hat{n} \cdot \vec{v}_1 \vec{S}_1 \cdot \vec{v}_2 - 75 \hat{n} \cdot \vec{S}_1 \hat{n} \cdot \vec{v}_2 \vec{S}_1 \cdot \vec{v}_2 - \frac{51}{4} \vec{S}_1 \cdot \vec{S}_1 (\hat{n} \cdot \vec{v}_2)^2 + \\
25 \vec{S}_1 \cdot \vec{S}_1 \hat{n} \cdot \vec{v}_1 \hat{n} \cdot \vec{v}_2 + \frac{15}{2} (\vec{S}_1 \cdot \vec{v}_2)^2 - 18 \vec{S}_1 \cdot \vec{v}_1 \vec{S}_1 \cdot \vec{v}_2 - 5 \vec{S}_1 \cdot \vec{S}_1 \vec{v}_1 \cdot \vec{v}_2 + \frac{5}{4} \vec{S}_1 \cdot \vec{S}_1 \vec{v}_2 \cdot \vec{v}_2 \Big) + \\
\left. \frac{90 \hat{n} \cdot \vec{S}_1 \hat{n} \cdot \vec{S}_1 \hat{n} \cdot \vec{v}_2 - 18 \vec{S}_1 \cdot \vec{S}_1 \hat{n} \cdot \vec{v}_2 + 4 \vec{S}_1^2 \hat{n} \cdot \vec{v}_2 - 18 \hat{n} \cdot \vec{S}_1 \vec{S}_1 \cdot \vec{v}_2 - 18 \hat{n} \cdot \vec{S}_1 \vec{S}_1 \cdot \vec{v}_2}{r^4} \right\}$$

{DiagS1CES2[3, 2, 27],

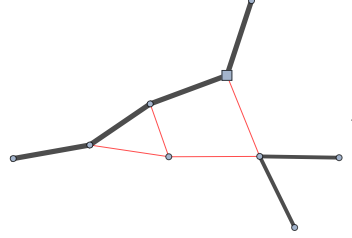

$$G^3 m_1 m_2 C_{ES^2 1} \left\{ \frac{1}{r^5} \left( \frac{63}{4} (\hat{n} \cdot \vec{S}_1)^2 (\hat{n} \cdot \vec{v}_1)^2 - 21 (\hat{n} \cdot \vec{S}_1)^2 \hat{n} \cdot \vec{v}_1 \hat{n} \cdot \vec{v}_2 - \frac{3}{4} \vec{v}_1 \cdot \vec{v}_1 (\hat{n} \cdot \vec{S}_1)^2 + \right. \right. \\
3 \vec{v}_1 \cdot \vec{v}_2 (\hat{n} \cdot \vec{S}_1)^2 - 6 \hat{n} \cdot \vec{S}_1 \hat{n} \cdot \vec{v}_1 \vec{S}_1 \cdot \vec{v}_1 + 6 \hat{n} \cdot \vec{S}_1 \hat{n} \cdot \vec{v}_1 \vec{S}_1 \cdot \vec{v}_2 - \frac{13}{4} \vec{S}_1 \cdot \vec{S}_1 (\hat{n} \cdot \vec{v}_1)^2 + \\
5 \vec{S}_1 \cdot \vec{S}_1 \hat{n} \cdot \vec{v}_1 \hat{n} \cdot \vec{v}_2 + \frac{1}{4} \vec{S}_1 \cdot \vec{S}_1 \vec{v}_1 \cdot \vec{v}_1 - \vec{S}_1 \cdot \vec{S}_1 \vec{v}_1 \cdot \vec{v}_2 \Big) + \left. \frac{2 \vec{S}_1 \cdot \vec{S}_1 \hat{n} \cdot \vec{v}_1 - 6 \hat{n} \cdot \vec{S}_1 \hat{n} \cdot \vec{S}_1 \hat{n} \cdot \vec{v}_1}{r^4} \right\}$$

{DiagS1CES2[3, 2, 28],

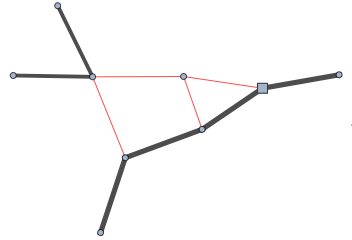

$$G^3 m_1 m_2 C_{ES^2 1} \left\{ \frac{1}{r^5} \left( \frac{39}{4} (\hat{n} \cdot \vec{S}_1)^2 (\hat{n} \cdot \vec{v}_1)^2 - 42 (\hat{n} \cdot \vec{S}_1)^2 \hat{n} \cdot \vec{v}_1 \hat{n} \cdot \vec{v}_2 - \frac{5}{4} \vec{v}_1 \cdot \vec{v}_1 (\hat{n} \cdot \vec{S}_1)^2 + 6 \vec{v}_1 \cdot \vec{v}_2 (\hat{n} \cdot \vec{S}_1)^2 - \right. \right. \\
6 \hat{n} \cdot \vec{S}_1 \hat{n} \cdot \vec{v}_1 \vec{S}_1 \cdot \vec{v}_1 + 15 \hat{n} \cdot \vec{S}_1 \hat{n} \cdot \vec{v}_2 \vec{S}_1 \cdot \vec{v}_1 + 12 \hat{n} \cdot \vec{S}_1 \hat{n} \cdot \vec{v}_1 \vec{S}_1 \cdot \vec{v}_2 - \frac{5}{4} \vec{S}_1 \cdot \vec{S}_1 (\hat{n} \cdot \vec{v}_1)^2 + 5 \vec{S}_1 \cdot \vec{S}_1 \hat{n} \cdot \vec{v}_1 \hat{n} \cdot \vec{v}_2 + \\
\frac{1}{2} (\vec{S}_1 \cdot \vec{v}_1)^2 - 3 \vec{S}_1 \cdot \vec{v}_1 \vec{S}_1 \cdot \vec{v}_2 + \frac{1}{4} \vec{S}_1 \cdot \vec{S}_1 \vec{v}_1 \cdot \vec{v}_1 - \vec{S}_1 \cdot \vec{S}_1 \vec{v}_1 \cdot \vec{v}_2 \Big) + \frac{1}{r^4} \left( -5 \hat{n} \cdot \vec{S}_1 \hat{n} \cdot \vec{S}_1 \hat{n} \cdot \vec{v}_1 + \vec{S}_1 \cdot \vec{S}_1 \hat{n} \cdot \vec{v}_1 + \right. \\
15 \hat{n} \cdot \vec{S}_1 \hat{n} \cdot \vec{S}_1 \hat{n} \cdot \vec{v}_2 + \hat{n} \cdot \vec{S}_1 \vec{S}_1 \cdot \vec{v}_1 - 3 \hat{n} \cdot \vec{S}_1 \vec{S}_1 \cdot \vec{v}_2 - 3 \vec{S}_1 \cdot \vec{S}_1 \hat{n} \cdot \vec{v}_2 + \hat{n} \cdot \vec{S}_1 \vec{S}_1 \cdot \vec{v}_1 - 3 \hat{n} \cdot \vec{S}_1 \vec{S}_1 \cdot \vec{v}_2 \Big) \Big\}$$

{DiagS1CES2[3, 2, 29],

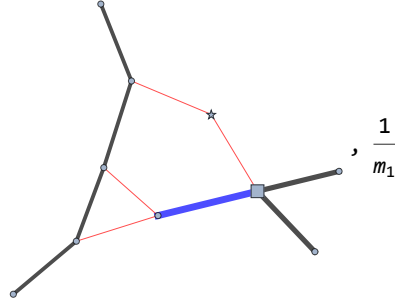

$$G^3 m_2^3 C_{ES^2 1} \left\{ \frac{1}{r^5} \left( -\frac{15}{4} (\hat{n} \cdot \vec{S}_1)^2 (\hat{n} \cdot \vec{v}_2)^2 + 7 (\hat{n} \cdot \vec{S}_1)^2 \hat{n} \cdot \vec{v}_1 \hat{n} \cdot \vec{v}_2 - \vec{v}_1 \cdot \vec{v}_2 (\hat{n} \cdot \vec{S}_1)^2 + \right. \right. \\ \left. \frac{3}{4} \vec{v}_2 \cdot \vec{v}_2 (\hat{n} \cdot \vec{S}_1)^2 - 2 \hat{n} \cdot \vec{S}_1 \hat{n} \cdot \vec{v}_2 \vec{S}_1 \cdot \vec{v}_1 - \frac{15}{4} \hat{n} \cdot \vec{S}_1 \hat{n} \cdot \vec{v}_1 \vec{S}_1 \cdot \vec{v}_2 + \frac{11}{4} \hat{n} \cdot \vec{S}_1 \hat{n} \cdot \vec{v}_2 \vec{S}_1 \cdot \vec{v}_2 + \right. \\ \left. \frac{5}{4} \vec{S}_1 \cdot \vec{S}_1 \hat{n} \cdot \vec{v}_1 \hat{n} \cdot \vec{v}_2 - \frac{1}{4} (\vec{S}_1 \cdot \vec{v}_2)^2 + \frac{3}{4} \vec{S}_1 \cdot \vec{v}_1 \vec{S}_1 \cdot \vec{v}_2 - \frac{1}{4} \vec{S}_1 \cdot \vec{S}_1 \vec{v}_1 \cdot \vec{v}_2 - \frac{1}{2} \vec{S}_1 \cdot \vec{S}_1 \vec{v}_2 \cdot \vec{v}_2 \right) + \\ \left. \frac{-2 \hat{n} \cdot \vec{S}_1 \hat{n} \cdot \vec{S}_1 \hat{n} \cdot \vec{v}_2 - \frac{1}{2} \vec{S}_1 \cdot \vec{S}_1 \hat{n} \cdot \vec{v}_2 + \frac{3}{4} \hat{n} \cdot \vec{S}_1 \vec{S}_1 \cdot \vec{v}_2 + \frac{3}{4} \hat{n} \cdot \vec{S}_1 \vec{S}_1 \cdot \vec{v}_2}{r^4} \right\}$$

{DiagS1CES2[3, 2, 30],

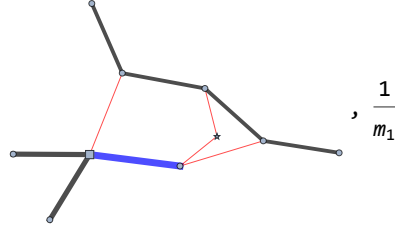

$$G^3 m_2^3 C_{ES^2 1} \left\{ \frac{1}{r^5} \left( -\frac{31}{12} (\hat{n} \cdot \vec{S}_1)^2 (\hat{n} \cdot \vec{v}_2)^2 + \frac{7}{12} (\hat{n} \cdot \vec{S}_1)^2 \hat{n} \cdot \vec{v}_1 \hat{n} \cdot \vec{v}_2 - \frac{1}{12} \vec{v}_1 \cdot \vec{v}_2 (\hat{n} \cdot \vec{S}_1)^2 + \frac{7}{12} \vec{v}_2 \cdot \vec{v}_2 (\hat{n} \cdot \vec{S}_1)^2 - \right. \right. \\ \left. \frac{1}{6} \hat{n} \cdot \vec{S}_1 \hat{n} \cdot \vec{v}_2 \vec{S}_1 \cdot \vec{v}_1 + \frac{10}{3} \hat{n} \cdot \vec{S}_1 \hat{n} \cdot \vec{v}_1 \vec{S}_1 \cdot \vec{v}_2 - \frac{11}{3} \hat{n} \cdot \vec{S}_1 \hat{n} \cdot \vec{v}_2 \vec{S}_1 \cdot \vec{v}_2 + \frac{73}{12} \vec{S}_1 \cdot \vec{S}_1 (\hat{n} \cdot \vec{v}_2)^2 - \right. \\ \left. \frac{55}{12} \vec{S}_1 \cdot \vec{S}_1 \hat{n} \cdot \vec{v}_1 \hat{n} \cdot \vec{v}_2 + \frac{7}{6} (\vec{S}_1 \cdot \vec{v}_2)^2 - \frac{2}{3} \vec{S}_1 \cdot \vec{v}_1 \vec{S}_1 \cdot \vec{v}_2 + \frac{11}{12} \vec{S}_1 \cdot \vec{S}_1 \vec{v}_1 \cdot \vec{v}_2 - \frac{23}{12} \vec{S}_1 \cdot \vec{S}_1 \vec{v}_2 \cdot \vec{v}_2 \right) + \\ \left. \frac{-\frac{1}{6} \hat{n} \cdot \vec{S}_1 \hat{n} \cdot \vec{S}_1 \hat{n} \cdot \vec{v}_2 + \frac{11}{6} \vec{S}_1 \cdot \vec{S}_1 \hat{n} \cdot \vec{v}_2 - \frac{2}{3} \hat{n} \cdot \vec{S}_1 \vec{S}_1 \cdot \vec{v}_2 - \frac{2}{3} \hat{n} \cdot \vec{S}_1 \vec{S}_1 \cdot \vec{v}_2}{r^4} \right\}$$

{DiagS1CES2[3, 2, 31],

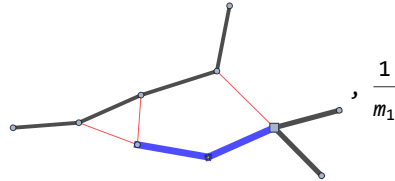

$$G^3 m_2^3 C_{ES^2 1} \left\{ \frac{1}{r^5} \left( -\frac{19}{3} (\hat{n} \cdot \vec{S}_1)^2 (\hat{n} \cdot \vec{v}_2)^2 + \frac{28}{3} (\hat{n} \cdot \vec{S}_1)^2 \hat{n} \cdot \vec{v}_1 \hat{n} \cdot \vec{v}_2 - \frac{4}{3} \vec{v}_1 \cdot \vec{v}_2 (\hat{n} \cdot \vec{S}_1)^2 + \frac{1}{3} \vec{v}_2 \cdot \vec{v}_2 (\hat{n} \cdot \vec{S}_1)^2 - \right. \right. \\ \left. \frac{8}{3} \hat{n} \cdot \vec{S}_1 \hat{n} \cdot \vec{v}_2 \vec{S}_1 \cdot \vec{v}_1 - \frac{5}{12} \hat{n} \cdot \vec{S}_1 \hat{n} \cdot \vec{v}_1 \vec{S}_1 \cdot \vec{v}_2 + \frac{31}{12} \hat{n} \cdot \vec{S}_1 \hat{n} \cdot \vec{v}_2 \vec{S}_1 \cdot \vec{v}_2 + \frac{19}{12} \vec{S}_1 \cdot \vec{S}_1 (\hat{n} \cdot \vec{v}_2)^2 - \right. \\ \left. \frac{1}{6} \hat{n} \cdot \vec{S}_1 \hat{n} \cdot \vec{S}_1 \hat{n} \cdot \vec{v}_2 + \frac{11}{6} \vec{S}_1 \cdot \vec{S}_1 \hat{n} \cdot \vec{v}_2 - \frac{2}{3} \hat{n} \cdot \vec{S}_1 \vec{S}_1 \cdot \vec{v}_2 - \frac{2}{3} \hat{n} \cdot \vec{S}_1 \vec{S}_1 \cdot \vec{v}_2 \right) + \\ \left. \frac{-\frac{1}{6} \hat{n} \cdot \vec{S}_1 \hat{n} \cdot \vec{S}_1 \hat{n} \cdot \vec{v}_2 + \frac{11}{6} \vec{S}_1 \cdot \vec{S}_1 \hat{n} \cdot \vec{v}_2 - \frac{2}{3} \hat{n} \cdot \vec{S}_1 \vec{S}_1 \cdot \vec{v}_2 - \frac{2}{3} \hat{n} \cdot \vec{S}_1 \vec{S}_1 \cdot \vec{v}_2}{r^4} \right\}$$

$$\left. \begin{aligned} & \frac{25}{12} \vec{S}_1 \cdot \vec{S}_1 \hat{n} \cdot \vec{v}_1 \hat{n} \cdot \vec{v}_2 - \frac{1}{12} \left( \vec{S}_1 \cdot \vec{v}_2 \right)^2 + \frac{1}{12} \vec{S}_1 \cdot \vec{v}_1 \vec{S}_1 \cdot \vec{v}_2 + \frac{5}{12} \vec{S}_1 \cdot \vec{S}_1 \vec{v}_1 \cdot \vec{v}_2 - \frac{5}{12} \vec{S}_1 \cdot \vec{S}_1 \vec{v}_2 \cdot \vec{v}_2 \right) + \\ & \left. - \frac{8}{3} \hat{n} \cdot \vec{S}_1 \hat{n} \cdot \vec{S}_1 \hat{n} \cdot \vec{v}_2 + \frac{5}{6} \vec{S}_1 \cdot \vec{S}_1 \hat{n} \cdot \vec{v}_2 + \frac{1}{12} \hat{n} \cdot \vec{S}_1 \vec{S}_1 \cdot \vec{v}_2 + \frac{1}{12} \hat{n} \cdot \vec{S}_1 \vec{S}_1 \cdot \vec{v}_2 \right) \Bigg\} \\ & r^4 \end{aligned}$$

{DiagS1CES2[3, 2, 32],

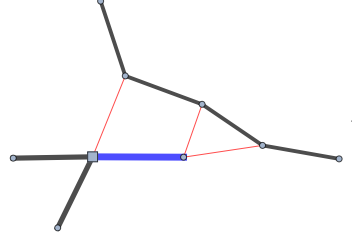

$$\begin{aligned} & \frac{1}{m_1} G^3 m_2^3 C_{ES^2 1} \left( \frac{-\left(\hat{n} \cdot \vec{a}_2\right) \left(\hat{n} \cdot \vec{S}_1\right)^2 + \frac{1}{2} \vec{S}_1 \cdot \vec{a}_2 \hat{n} \cdot \vec{S}_1 - \frac{1}{2} \vec{S}_1 \cdot \vec{S}_1 \hat{n} \cdot \vec{a}_2}{r^4} + \frac{1}{r^5} \right. \\ & \left( -\frac{25}{2} \left(\hat{n} \cdot \vec{S}_1\right)^2 \left(\hat{n} \cdot \vec{v}_2\right)^2 - \frac{3}{2} \left(\hat{n} \cdot \vec{S}_1\right)^2 \hat{n} \cdot \vec{v}_1 \hat{n} \cdot \vec{v}_2 + \frac{5}{2} \vec{v}_1 \cdot \vec{v}_1 \left(\hat{n} \cdot \vec{S}_1\right)^2 + \vec{v}_1 \cdot \vec{v}_2 \left(\hat{n} \cdot \vec{S}_1\right)^2 + \right. \\ & \frac{5}{4} \vec{v}_2 \cdot \vec{v}_2 \left(\hat{n} \cdot \vec{S}_1\right)^2 - \frac{17}{4} \hat{n} \cdot \vec{S}_1 \hat{n} \cdot \vec{v}_1 \vec{S}_1 \cdot \vec{v}_1 + \frac{11}{2} \hat{n} \cdot \vec{S}_1 \hat{n} \cdot \vec{v}_2 \vec{S}_1 \cdot \vec{v}_1 - \frac{1}{2} \hat{n} \cdot \vec{S}_1 \hat{n} \cdot \vec{v}_1 \vec{S}_1 \cdot \vec{v}_2 + \\ & \frac{13}{2} \hat{n} \cdot \vec{S}_1 \hat{n} \cdot \vec{v}_2 \vec{S}_1 \cdot \vec{v}_2 + \frac{3}{4} \vec{S}_1 \cdot \vec{S}_1 \left(\hat{n} \cdot \vec{v}_1\right)^2 - 3 \vec{S}_1 \cdot \vec{S}_1 \left(\hat{n} \cdot \vec{v}_2\right)^2 + \frac{11}{2} \vec{S}_1 \cdot \vec{S}_1 \hat{n} \cdot \vec{v}_1 \hat{n} \cdot \vec{v}_2 + \\ & \left. \left. \frac{1}{2} \left(\vec{S}_1 \cdot \vec{v}_1\right)^2 - \frac{1}{2} \left(\vec{S}_1 \cdot \vec{v}_2\right)^2 - \vec{S}_1 \cdot \vec{v}_1 \vec{S}_1 \cdot \vec{v}_2 - 2 \vec{S}_1 \cdot \vec{S}_1 \vec{v}_1 \cdot \vec{v}_1 - 2 \vec{S}_1 \cdot \vec{S}_1 \vec{v}_1 \cdot \vec{v}_2 - \frac{9}{4} \vec{S}_1 \cdot \vec{S}_1 \vec{v}_2 \cdot \vec{v}_2 \right) \right\} \end{aligned}$$

{DiagS1CES2[3, 3, 1],

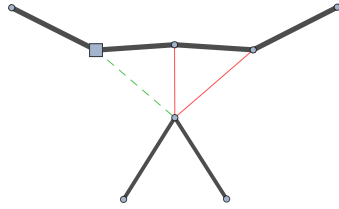

$$G^3 m_1 m_2 C_{ES^2 1} \left( \frac{3 \vec{v}_1 \cdot \vec{v}_2 \left(\hat{n} \cdot \vec{S}_1\right)^2 - \vec{S}_1 \cdot \vec{S}_1 \vec{v}_1 \cdot \vec{v}_2}{r^5} + \frac{-\left(\hat{n} \cdot \vec{S}_1\right) \frac{1}{S_1} \cdot \vec{v}_2 + 2 \vec{S}_1 \cdot \vec{S}_1 \hat{n} \cdot \vec{v}_2 - \hat{n} \cdot \vec{S}_1 \vec{S}_1 \cdot \vec{v}_2}{r^4} \right) \Bigg\}$$

{DiagS1CES2[3, 3, 2],

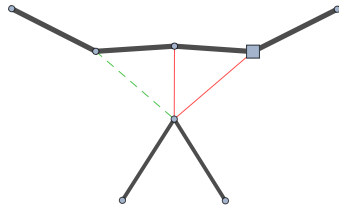

$$, \frac{G^3 m_1 m_2 C_{ES^2 1} \left( 6 \vec{v}_1 \cdot \vec{v}_2 \left(\hat{n} \cdot \vec{S}_1\right)^2 - 2 \vec{S}_1 \cdot \vec{S}_1 \vec{v}_1 \cdot \vec{v}_2 \right)}{r^5} \Bigg\}$$

{DiagS1CES2[3, 3, 3],

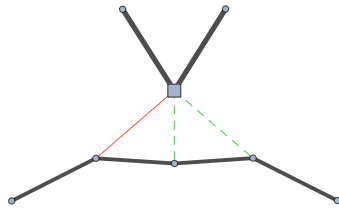



$$\frac{G^3 m_2^3 C_{ES^2 1} \left( -14 \vec{v}_2 \cdot \vec{v}_2 \left( \hat{n} \cdot \vec{S}_1 \right)^2 + 28 \hat{n} \cdot \vec{S}_1 \hat{n} \cdot \vec{v}_2 \vec{S}_1 \cdot \vec{v}_2 - 28 \vec{S}_1 \cdot \vec{S}_1 \left( \hat{n} \cdot \vec{v}_2 \right)^2 - 14 \left( \vec{S}_1 \cdot \vec{v}_2 \right)^2 + 28 \vec{S}_1 \cdot \vec{S}_1 \vec{v}_2 \cdot \vec{v}_2 \right)}{m_1 r^5}$$

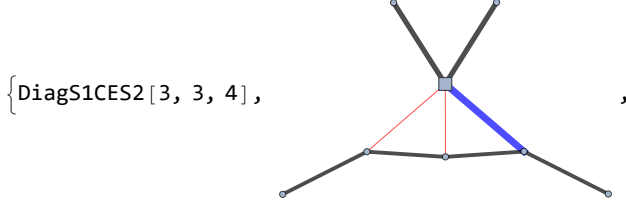

$$\frac{G^3 m_2^3 C_{ES^2 1} \left( 30 \vec{v}_2 \cdot \vec{v}_2 \left( \hat{n} \cdot \vec{S}_1 \right)^2 - 30 \hat{n} \cdot \vec{S}_1 \hat{n} \cdot \vec{v}_2 \vec{S}_1 \cdot \vec{v}_2 + 26 \vec{S}_1 \cdot \vec{S}_1 \left( \hat{n} \cdot \vec{v}_2 \right)^2 + 9 \left( \vec{S}_1 \cdot \vec{v}_2 \right)^2 - 17 \vec{S}_1 \cdot \vec{S}_1 \vec{v}_2 \cdot \vec{v}_2 \right)}{m_1 r^5}$$

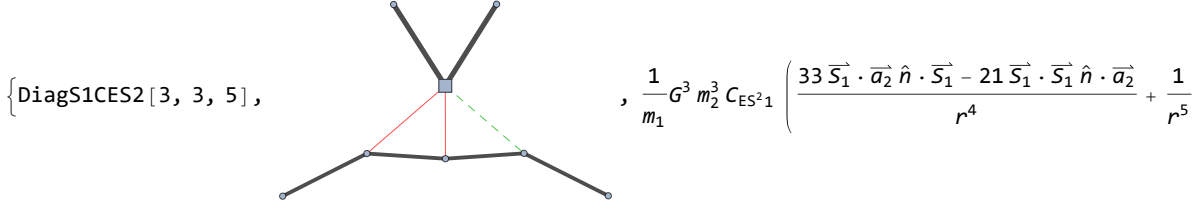

$$\left( 87 \vec{v}_1 \cdot \vec{v}_2 \left( \hat{n} \cdot \vec{S}_1 \right)^2 - 6 \hat{n} \cdot \vec{S}_1 \hat{n} \cdot \vec{v}_2 \vec{S}_1 \cdot \vec{v}_1 - 63 \hat{n} \cdot \vec{S}_1 \hat{n} \cdot \vec{v}_1 \vec{S}_1 \cdot \vec{v}_2 + 105 \hat{n} \cdot \vec{S}_1 \hat{n} \cdot \vec{v}_2 \vec{S}_1 \cdot \vec{v}_2 - 85 \vec{S}_1 \cdot \vec{S}_1 \left( \hat{n} \cdot \vec{v}_2 \right)^2 + 57 \vec{S}_1 \cdot \vec{S}_1 \hat{n} \cdot \vec{v}_1 \hat{n} \cdot \vec{v}_2 - 21 \left( \vec{S}_1 \cdot \vec{v}_2 \right)^2 + 15 \vec{S}_1 \cdot \vec{v}_1 \vec{S}_1 \cdot \vec{v}_2 - 56 \vec{S}_1 \cdot \vec{S}_1 \vec{v}_1 \cdot \vec{v}_2 + 21 \vec{S}_1 \cdot \vec{S}_1 \vec{v}_2 \cdot \vec{v}_2 \right)$$

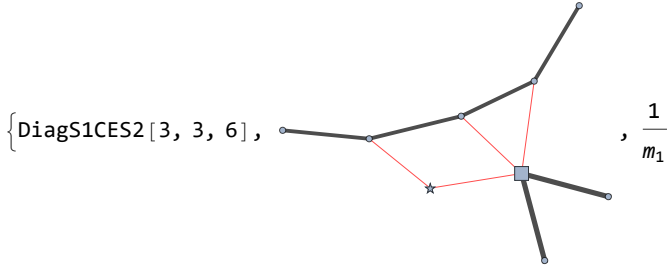

$$G^3 m_2^3 C_{ES^2 1} \left( \frac{1}{r^5} \left( -\frac{315}{4} \left( \hat{n} \cdot \vec{S}_1 \right)^2 \left( \hat{n} \cdot \vec{v}_2 \right)^2 + \frac{945}{8} \left( \hat{n} \cdot \vec{S}_1 \right)^2 \hat{n} \cdot \vec{v}_1 \hat{n} \cdot \vec{v}_2 - \frac{135}{8} \vec{v}_1 \cdot \vec{v}_2 \left( \hat{n} \cdot \vec{S}_1 \right)^2 - \frac{135}{4} \hat{n} \cdot \vec{S}_1 \hat{n} \cdot \vec{v}_2 \vec{S}_1 \cdot \vec{v}_1 - \frac{135}{4} \hat{n} \cdot \vec{S}_1 \hat{n} \cdot \vec{v}_1 \vec{S}_1 \cdot \vec{v}_2 + 45 \hat{n} \cdot \vec{S}_1 \hat{n} \cdot \vec{v}_2 \vec{S}_1 \cdot \vec{v}_2 + \frac{33}{4} \vec{S}_1 \cdot \vec{S}_1 \left( \hat{n} \cdot \vec{v}_2 \right)^2 - \frac{75}{8} \vec{S}_1 \cdot \vec{S}_1 \hat{n} \cdot \vec{v}_1 \hat{n} \cdot \vec{v}_2 - \frac{9}{2} \left( \vec{S}_1 \cdot \vec{v}_2 \right)^2 + \frac{27}{4} \vec{S}_1 \cdot \vec{v}_1 \vec{S}_1 \cdot \vec{v}_2 + \frac{15}{8} \vec{S}_1 \cdot \vec{S}_1 \vec{v}_1 \cdot \vec{v}_2 + \frac{3}{2} \vec{S}_1 \cdot \vec{S}_1 \vec{v}_2 \cdot \vec{v}_2 \right) + \frac{-\frac{135}{4} \hat{n} \cdot \vec{S}_1 \hat{n} \cdot \vec{S}_1 \hat{n} \cdot \vec{v}_2 + \frac{27}{4} \vec{S}_1 \cdot \vec{S}_1 \hat{n} \cdot \vec{v}_2 - \frac{3}{2} \vec{S}_1^2 \hat{n} \cdot \vec{v}_2 + \frac{27}{4} \hat{n} \cdot \vec{S}_1 \vec{S}_1 \cdot \vec{v}_2 + \frac{27}{4} \hat{n} \cdot \vec{S}_1 \vec{S}_1 \cdot \vec{v}_2}{r^4} \right)$$

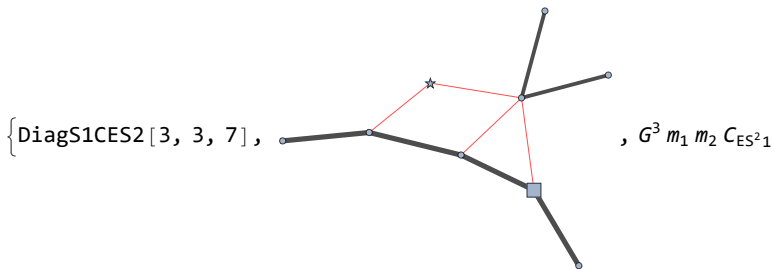

$$\left\{ \frac{1}{r^5} \left( -\frac{9}{2} (\hat{n} \cdot \vec{S}_1)^2 (\hat{n} \cdot \vec{v}_1)^2 + \frac{21}{4} (\hat{n} \cdot \vec{S}_1)^2 \hat{n} \cdot \vec{v}_1 \hat{n} \cdot \vec{v}_2 - \frac{3}{4} \vec{v}_1 \cdot \vec{v}_2 (\hat{n} \cdot \vec{S}_1)^2 + \frac{3}{2} \hat{n} \cdot \vec{S}_1 \hat{n} \cdot \vec{v}_1 \vec{S}_1 \cdot \vec{v}_1 - \frac{3}{2} \hat{n} \cdot \vec{S}_1 \hat{n} \cdot \vec{v}_1 \right. \right. \\ \left. \left. \vec{S}_1 \cdot \vec{v}_2 + \vec{S}_1 \cdot \vec{S}_1 (\hat{n} \cdot \vec{v}_1)^2 - \frac{5}{4} \vec{S}_1 \cdot \vec{S}_1 \hat{n} \cdot \vec{v}_1 \hat{n} \cdot \vec{v}_2 + \frac{1}{4} \vec{S}_1 \cdot \vec{S}_1 \vec{v}_1 \cdot \vec{v}_2 \right) + \frac{\frac{3}{2} \hat{n} \cdot \vec{S}_1 \hat{n} \cdot \vec{S}_1 \hat{n} \cdot \vec{v}_1 - \frac{1}{2} \vec{S}_1 \cdot \vec{S}_1 \hat{n} \cdot \vec{v}_1}{r^4} \right\}$$

{DiagS1CES2[3, 3, 8],

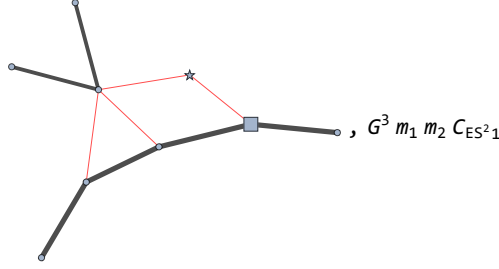

,  $G^3 m_1 m_2 C_{ES^2 1}$

$$\left\{ \frac{1}{r^5} \left( -\frac{3}{4} (\hat{n} \cdot \vec{S}_1)^2 (\hat{n} \cdot \vec{v}_1)^2 + \frac{21}{8} (\hat{n} \cdot \vec{S}_1)^2 \hat{n} \cdot \vec{v}_1 \hat{n} \cdot \vec{v}_2 - \frac{3}{8} \vec{v}_1 \cdot \vec{v}_2 (\hat{n} \cdot \vec{S}_1)^2 + \frac{1}{2} \hat{n} \cdot \vec{S}_1 \hat{n} \cdot \vec{v}_1 \vec{S}_1 \cdot \vec{v}_1 - \frac{5}{4} \hat{n} \cdot \vec{S}_1 \hat{n} \cdot \vec{v}_2 \right. \right. \\ \left. \left. \vec{S}_1 \cdot \vec{v}_1 - \frac{3}{4} \hat{n} \cdot \vec{S}_1 \hat{n} \cdot \vec{v}_1 \vec{S}_1 \cdot \vec{v}_2 - \frac{1}{4} \vec{S}_1 \cdot \vec{S}_1 (\hat{n} \cdot \vec{v}_1)^2 + \frac{5}{8} \vec{S}_1 \cdot \vec{S}_1 \hat{n} \cdot \vec{v}_1 \hat{n} \cdot \vec{v}_2 + \frac{1}{4} \vec{S}_1 \cdot \vec{v}_1 \vec{S}_1 \cdot \vec{v}_2 - \frac{1}{8} \vec{S}_1 \cdot \vec{S}_1 \vec{v}_1 \cdot \vec{v}_2 \right) + \right. \\ \left. \frac{\frac{1}{2} \hat{n} \cdot \vec{S}_1 \hat{n} \cdot \vec{S}_1 \hat{n} \cdot \vec{v}_1 + \frac{1}{2} \vec{S}_1 \cdot \vec{S}_1 \hat{n} \cdot \vec{v}_1 - \frac{5}{4} \hat{n} \cdot \vec{S}_1 \hat{n} \cdot \vec{S}_1 \hat{n} \cdot \vec{v}_2 + \frac{1}{4} \hat{n} \cdot \vec{S}_1 \vec{S}_1 \cdot \vec{v}_2 - \frac{3}{4} \vec{S}_1 \cdot \vec{S}_1 \hat{n} \cdot \vec{v}_2 + \frac{1}{4} \hat{n} \cdot \vec{S}_1 \vec{S}_1 \cdot \vec{v}_2}{r^4} \right\}$$

{DiagS1CES2[3, 3, 9],

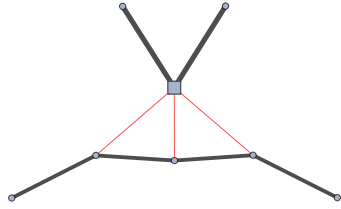

,  $\frac{1}{m_1}$

$$G^3 m_2^3 C_{ES^2 1} \left( \frac{\vec{S}_1 \cdot \vec{S}_1 \hat{n} \cdot \vec{a}_2}{2 r^4} + \frac{1}{r^5} \left( \frac{1}{8} \vec{v}_1 \cdot \vec{v}_1 (\hat{n} \cdot \vec{S}_1)^2 - \frac{405}{8} \vec{v}_2 \cdot \vec{v}_2 (\hat{n} \cdot \vec{S}_1)^2 - \frac{1}{4} \hat{n} \cdot \vec{S}_1 \hat{n} \cdot \vec{v}_1 \vec{S}_1 \cdot \vec{v}_1 - \right. \right. \\ \left. \left. \frac{5}{2} \hat{n} \cdot \vec{S}_1 \hat{n} \cdot \vec{v}_2 \vec{S}_1 \cdot \vec{v}_1 + \frac{3}{4} \vec{S}_1 \cdot \vec{S}_1 (\hat{n} \cdot \vec{v}_1)^2 + \frac{7}{2} \vec{S}_1 \cdot \vec{S}_1 (\hat{n} \cdot \vec{v}_2)^2 - \frac{5}{2} \vec{S}_1 \cdot \vec{S}_1 \hat{n} \cdot \vec{v}_1 \hat{n} \cdot \vec{v}_2 + \right. \right. \\ \left. \left. \frac{1}{4} (\vec{S}_1 \cdot \vec{v}_1)^2 + \frac{1}{2} \vec{S}_1 \cdot \vec{v}_1 \vec{S}_1 \cdot \vec{v}_2 - \frac{1}{8} \vec{S}_1 \cdot \vec{S}_1 \vec{v}_1 \cdot \vec{v}_1 + \frac{1}{2} \vec{S}_1 \cdot \vec{S}_1 \vec{v}_1 \cdot \vec{v}_2 + \frac{131}{8} \vec{S}_1 \cdot \vec{S}_1 \vec{v}_2 \cdot \vec{v}_2 \right) \right)$$

{DiagS1CES2[3, 3, 10],

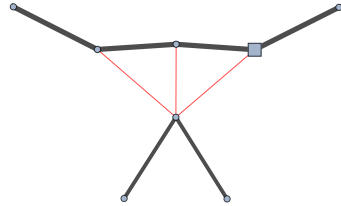

,  $G^3 m_1 m_2 C_{ES^2 1}$

$$\left( \frac{\frac{1}{2} \vec{S}_1 \cdot \vec{a}_1 \hat{n} \cdot \vec{S}_1 + \frac{1}{2} \hat{n} \cdot \vec{S}_1 \vec{S}_1 \cdot \vec{v}_1 - \vec{S}_1 \cdot \vec{S}_1 \hat{n} \cdot \vec{v}_1 + \frac{1}{2} \hat{n} \cdot \vec{S}_1 \vec{S}_1 \cdot \vec{v}_1}{r^4} + \frac{1}{r^5} \left( -\frac{27}{8} \vec{v}_1 \cdot \vec{v}_1 (\hat{n} \cdot \vec{S}_1)^2 - \frac{81}{8} \vec{v}_2 \cdot \vec{v}_2 (\hat{n} \cdot \vec{S}_1)^2 + \right. \right.$$

$$\left\{ \frac{3}{4} \hat{n} \cdot \vec{S}_1 \hat{n} \cdot \vec{v}_1 \vec{S}_1 \cdot \vec{v}_1 - \frac{3}{4} \vec{S}_1 \cdot \vec{S}_1 (\hat{n} \cdot \vec{v}_1)^2 - \frac{1}{4} (\vec{S}_1 \cdot \vec{v}_1)^2 + \frac{11}{8} \vec{S}_1 \cdot \vec{S}_1 \vec{v}_1 \cdot \vec{v}_1 + \frac{27}{8} \vec{S}_1 \cdot \vec{S}_1 \vec{v}_2 \cdot \vec{v}_2 \right\} + \frac{S_1^2}{2 r^3} \Bigg\}$$

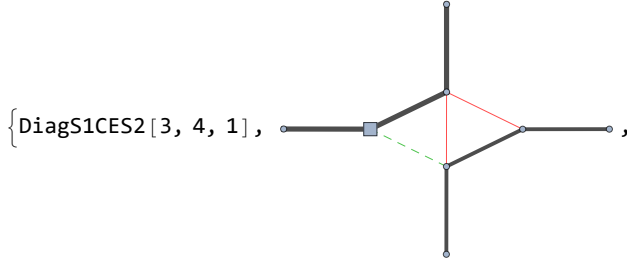

$$G^3 m_2^2 C_{ES^2 1} \left\{ \frac{6 \vec{v}_1 \cdot \vec{v}_2 (\hat{n} \cdot \vec{S}_1)^2 - 2 \vec{S}_1 \cdot \vec{S}_1 \vec{v}_1 \cdot \vec{v}_2}{r^5} + \frac{-2 \hat{n} \cdot \vec{S}_1 \vec{S}_1 \cdot \vec{v}_2 + 4 \vec{S}_1 \cdot \vec{S}_1 \hat{n} \cdot \vec{v}_2 - 2 \hat{n} \cdot \vec{S}_1 \vec{S}_1 \cdot \vec{v}_2}{r^4} \right\}$$

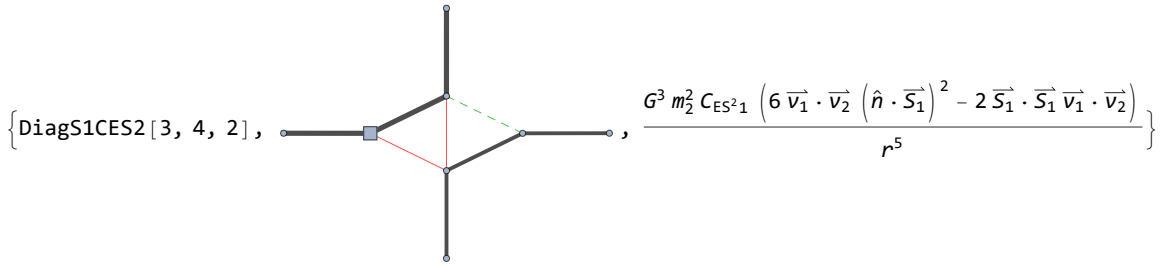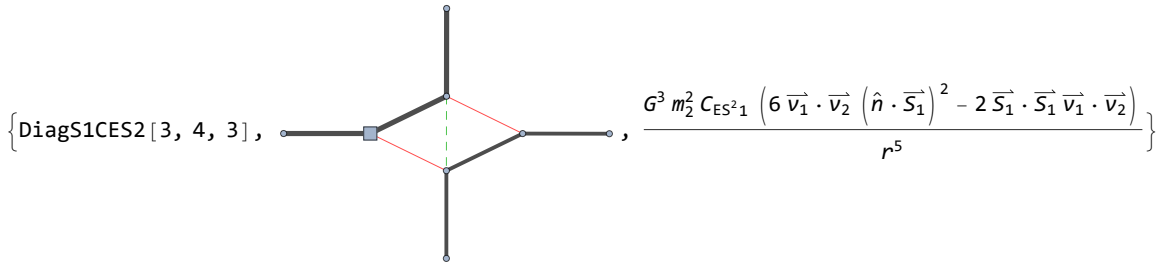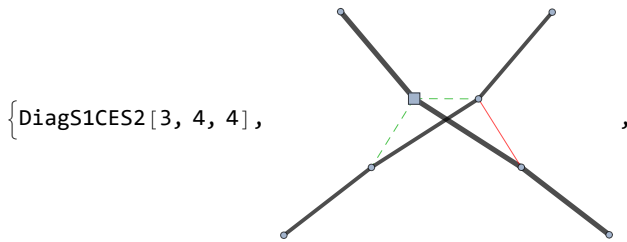

$$\frac{G^3 m_2^2 C_{ES^2 1} \left( -4 \vec{v}_2 \cdot \vec{v}_2 (\hat{n} \cdot \vec{S}_1)^2 + 8 \hat{n} \cdot \vec{S}_1 \hat{n} \cdot \vec{v}_2 \vec{S}_1 \cdot \vec{v}_2 - 8 \vec{S}_1 \cdot \vec{S}_1 (\hat{n} \cdot \vec{v}_2)^2 - 4 (\vec{S}_1 \cdot \vec{v}_2)^2 + 8 \vec{S}_1 \cdot \vec{S}_1 \vec{v}_2 \cdot \vec{v}_2 \right)}{r^5} \Bigg\}$$

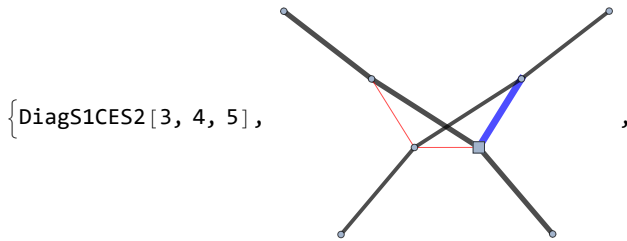

$$\frac{G^3 m_2^2 C_{ES^2 1} \left( 8 \vec{v}_2 \cdot \vec{v}_2 \left( \hat{n} \cdot \vec{S}_1 \right)^2 - 8 \hat{n} \cdot \vec{S}_1 \hat{n} \cdot \vec{v}_2 \vec{S}_1 \cdot \vec{v}_2 + 8 \vec{S}_1 \cdot \vec{S}_1 \left( \hat{n} \cdot \vec{v}_2 \right)^2 + 3 \left( \vec{S}_1 \cdot \vec{v}_2 \right)^2 - 5 \vec{S}_1 \cdot \vec{S}_1 \vec{v}_2 \cdot \vec{v}_2 \right)}{r^5}$$

{DiagS1CES2[3, 4, 6],

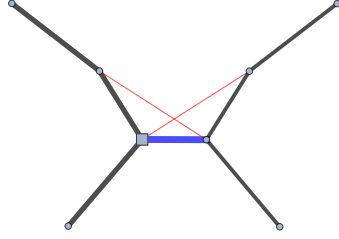

,

$$\frac{G^3 m_2^2 C_{ES^2 1} \left( -24 \vec{v}_2 \cdot \vec{v}_2 \left( \hat{n} \cdot \vec{S}_1 \right)^2 + 24 \hat{n} \cdot \vec{S}_1 \hat{n} \cdot \vec{v}_2 \vec{S}_1 \cdot \vec{v}_2 - 24 \vec{S}_1 \cdot \vec{S}_1 \left( \hat{n} \cdot \vec{v}_2 \right)^2 - 9 \left( \vec{S}_1 \cdot \vec{v}_2 \right)^2 + 15 \vec{S}_1 \cdot \vec{S}_1 \vec{v}_2 \cdot \vec{v}_2 \right)}{r^5}$$

{DiagS1CES2[3, 4, 7],

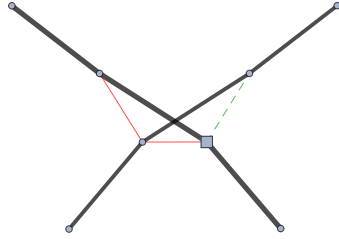

$$, G^3 m_2^2 C_{ES^2 1} \left( \frac{14 \vec{S}_1 \cdot \vec{a}_2 \hat{n} \cdot \vec{S}_1 - 10 \vec{S}_1 \cdot \vec{S}_1 \hat{n} \cdot \vec{a}_2}{r^4} + \frac{1}{r^5} \right)$$

$$\left( 36 \vec{v}_1 \cdot \vec{v}_2 \left( \hat{n} \cdot \vec{S}_1 \right)^2 - 2 \hat{n} \cdot \vec{S}_1 \hat{n} \cdot \vec{v}_2 \vec{S}_1 \cdot \vec{v}_1 - 36 \hat{n} \cdot \vec{S}_1 \hat{n} \cdot \vec{v}_1 \vec{S}_1 \cdot \vec{v}_2 + 46 \hat{n} \cdot \vec{S}_1 \hat{n} \cdot \vec{v}_2 \vec{S}_1 \cdot \vec{v}_2 - 42 \vec{S}_1 \cdot \vec{S}_1 \left( \hat{n} \cdot \vec{v}_2 \right)^2 + 34 \vec{S}_1 \cdot \vec{S}_1 \hat{n} \cdot \vec{v}_1 \hat{n} \cdot \vec{v}_2 - 10 \left( \vec{S}_1 \cdot \vec{v}_2 \right)^2 + 8 \vec{S}_1 \cdot \vec{v}_1 \vec{S}_1 \cdot \vec{v}_2 - 24 \vec{S}_1 \cdot \vec{S}_1 \vec{v}_1 \cdot \vec{v}_2 + 10 \vec{S}_1 \cdot \vec{S}_1 \vec{v}_2 \cdot \vec{v}_2 \right)$$

{DiagS1CES2[3, 4, 8],

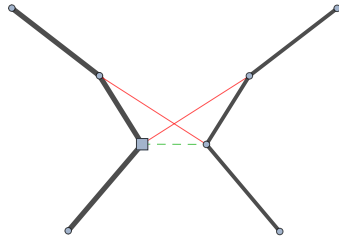

$$, G^3 m_2^2 C_{ES^2 1} \left( \frac{14 \vec{S}_1 \cdot \vec{a}_2 \hat{n} \cdot \vec{S}_1 - 10 \vec{S}_1 \cdot \vec{S}_1 \hat{n} \cdot \vec{a}_2}{r^4} + \frac{1}{r^5} \right)$$

$$\left( 36 \vec{v}_1 \cdot \vec{v}_2 \left( \hat{n} \cdot \vec{S}_1 \right)^2 - 2 \hat{n} \cdot \vec{S}_1 \hat{n} \cdot \vec{v}_2 \vec{S}_1 \cdot \vec{v}_1 - 44 \hat{n} \cdot \vec{S}_1 \hat{n} \cdot \vec{v}_1 \vec{S}_1 \cdot \vec{v}_2 + 54 \hat{n} \cdot \vec{S}_1 \hat{n} \cdot \vec{v}_2 \vec{S}_1 \cdot \vec{v}_2 - 46 \vec{S}_1 \cdot \vec{S}_1 \left( \hat{n} \cdot \vec{v}_2 \right)^2 + 38 \vec{S}_1 \cdot \vec{S}_1 \hat{n} \cdot \vec{v}_1 \hat{n} \cdot \vec{v}_2 - 10 \left( \vec{S}_1 \cdot \vec{v}_2 \right)^2 + 8 \vec{S}_1 \cdot \vec{v}_1 \vec{S}_1 \cdot \vec{v}_2 - 24 \vec{S}_1 \cdot \vec{S}_1 \vec{v}_1 \cdot \vec{v}_2 + 10 \vec{S}_1 \cdot \vec{S}_1 \vec{v}_2 \cdot \vec{v}_2 \right)$$

{DiagS1CES2[3, 4, 9],

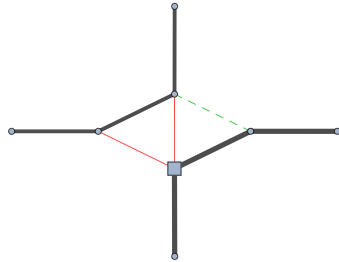

$$, \frac{G^3 m_2^2 C_{ES^2 1} \left( 48 \vec{v}_1 \cdot \vec{v}_2 \left( \hat{n} \cdot \vec{S}_1 \right)^2 - 16 \vec{S}_1 \cdot \vec{S}_1 \vec{v}_1 \cdot \vec{v}_2 \right)}{r^5}$$

{DiagS1CES2[3, 4, 10],

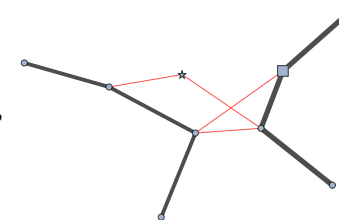

$$, G^3 m_2^2 C_{ES^2 1}$$

$$\left\{ \frac{1}{r^5} \left( -\frac{9}{2} (\hat{n} \cdot \vec{S}_1)^2 (\hat{n} \cdot \vec{v}_2)^2 + \frac{21}{4} (\hat{n} \cdot \vec{S}_1)^2 \hat{n} \cdot \vec{v}_1 \hat{n} \cdot \vec{v}_2 - \frac{3}{4} \vec{v}_1 \cdot \vec{v}_2 (\hat{n} \cdot \vec{S}_1)^2 - \frac{3}{2} \hat{n} \cdot \vec{S}_1 \hat{n} \cdot \vec{v}_2 \vec{S}_1 \cdot \vec{v}_1 + \frac{3}{2} \hat{n} \cdot \vec{S}_1 \hat{n} \cdot \vec{v}_2 \right. \right. \\ \left. \left. \vec{S}_1 \cdot \vec{v}_2 + \vec{S}_1 \cdot \vec{S}_1 (\hat{n} \cdot \vec{v}_2)^2 - \frac{5}{4} \vec{S}_1 \cdot \vec{S}_1 \hat{n} \cdot \vec{v}_1 \hat{n} \cdot \vec{v}_2 + \frac{1}{4} \vec{S}_1 \cdot \vec{S}_1 \vec{v}_1 \cdot \vec{v}_2 \right) + \frac{\frac{1}{2} \vec{S}_1 \cdot \vec{S}_1 \hat{n} \cdot \vec{v}_2 - \frac{3}{2} \hat{n} \cdot \vec{S}_1 \hat{n} \cdot \vec{S}_1 \hat{n} \cdot \vec{v}_2}{r^4} \right\}$$

{DiagS1CES2[3, 4, 11],

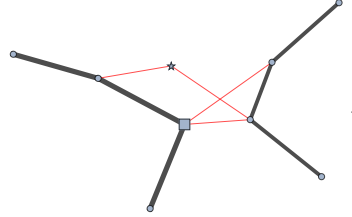

,

$$G^3 m_2^2 C_{ES^2_1} \left\{ \frac{1}{r^5} \left( -36 (\hat{n} \cdot \vec{S}_1)^2 (\hat{n} \cdot \vec{v}_1)^2 + 42 (\hat{n} \cdot \vec{S}_1)^2 \hat{n} \cdot \vec{v}_1 \hat{n} \cdot \vec{v}_2 - 6 \vec{v}_1 \cdot \vec{v}_2 (\hat{n} \cdot \vec{S}_1)^2 + 12 \hat{n} \cdot \vec{S}_1 \hat{n} \cdot \vec{v}_1 \vec{S}_1 \cdot \vec{v}_1 - \right. \right. \\ \left. \left. 12 \hat{n} \cdot \vec{S}_1 \hat{n} \cdot \vec{v}_1 \vec{S}_1 \cdot \vec{v}_2 + 8 \vec{S}_1 \cdot \vec{S}_1 (\hat{n} \cdot \vec{v}_1)^2 - 10 \vec{S}_1 \cdot \vec{S}_1 \hat{n} \cdot \vec{v}_1 \hat{n} \cdot \vec{v}_2 + 2 \vec{S}_1 \cdot \vec{S}_1 \vec{v}_1 \cdot \vec{v}_2 \right) + \right. \\ \left. \frac{12 \hat{n} \cdot \vec{S}_1 \hat{n} \cdot \vec{S}_1 \hat{n} \cdot \vec{v}_1 - 6 \vec{S}_1 \cdot \vec{S}_1 \hat{n} \cdot \vec{v}_1 + \vec{S}_1^2 \hat{n} \cdot \vec{v}_1}{r^4} \right\}$$

{DiagS1CES2[3, 4, 12],

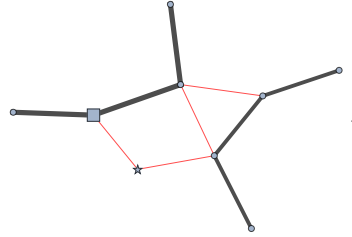

,  $G^3 m_2^2 C_{ES^2_1}$

$$\left\{ \frac{1}{r^5} \left( -\frac{3}{2} (\hat{n} \cdot \vec{S}_1)^2 (\hat{n} \cdot \vec{v}_1)^2 + \frac{21}{4} (\hat{n} \cdot \vec{S}_1)^2 \hat{n} \cdot \vec{v}_1 \hat{n} \cdot \vec{v}_2 - \frac{3}{4} \vec{v}_1 \cdot \vec{v}_2 (\hat{n} \cdot \vec{S}_1)^2 + \hat{n} \cdot \vec{S}_1 \hat{n} \cdot \vec{v}_1 \vec{S}_1 \cdot \vec{v}_1 - \frac{5}{2} \hat{n} \cdot \vec{S}_1 \hat{n} \cdot \vec{v}_2 \right. \right. \\ \left. \left. \vec{S}_1 \cdot \vec{v}_1 - \frac{3}{2} \hat{n} \cdot \vec{S}_1 \hat{n} \cdot \vec{v}_1 \vec{S}_1 \cdot \vec{v}_2 - \frac{1}{2} \vec{S}_1 \cdot \vec{S}_1 (\hat{n} \cdot \vec{v}_1)^2 + \frac{5}{4} \vec{S}_1 \cdot \vec{S}_1 \hat{n} \cdot \vec{v}_1 \hat{n} \cdot \vec{v}_2 + \frac{1}{2} \vec{S}_1 \cdot \vec{v}_1 \vec{S}_1 \cdot \vec{v}_2 - \frac{1}{4} \vec{S}_1 \cdot \vec{S}_1 \vec{v}_1 \cdot \vec{v}_2 \right) + \right. \\ \left. \frac{\hat{n} \cdot \vec{S}_1 \hat{n} \cdot \vec{S}_1 \hat{n} \cdot \vec{v}_1 + \vec{S}_1 \cdot \vec{S}_1 \hat{n} \cdot \vec{v}_1 - \frac{5}{2} \hat{n} \cdot \vec{S}_1 \hat{n} \cdot \vec{S}_1 \hat{n} \cdot \vec{v}_2 + \frac{1}{2} \hat{n} \cdot \vec{S}_1 \vec{S}_1 \cdot \vec{v}_2 - \frac{3}{2} \vec{S}_1 \cdot \vec{S}_1 \hat{n} \cdot \vec{v}_2 + \frac{1}{2} \hat{n} \cdot \vec{S}_1 \vec{S}_1 \cdot \vec{v}_2}{r^4} \right\}$$

{DiagS1CES2[3, 4, 13],

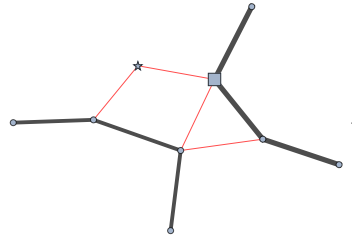

,

$$G^3 m_2^2 C_{ES^2_1} \left\{ \frac{1}{r^5} \left( -24 (\hat{n} \cdot \vec{S}_1)^2 (\hat{n} \cdot \vec{v}_2)^2 + 42 (\hat{n} \cdot \vec{S}_1)^2 \hat{n} \cdot \vec{v}_1 \hat{n} \cdot \vec{v}_2 - 6 \vec{v}_1 \cdot \vec{v}_2 (\hat{n} \cdot \vec{S}_1)^2 - \right. \right.$$

$$12 \hat{n} \cdot \vec{S}_1 \hat{n} \cdot \vec{v}_2 \vec{S}_1 \cdot \vec{v}_1 - 15 \hat{n} \cdot \vec{S}_1 \hat{n} \cdot \vec{v}_1 \vec{S}_1 \cdot \vec{v}_2 + 15 \hat{n} \cdot \vec{S}_1 \hat{n} \cdot \vec{v}_2 \vec{S}_1 \cdot \vec{v}_2 + \vec{S}_1 \cdot \vec{S}_1 (\hat{n} \cdot \vec{v}_2)^2 - \frac{3}{2} (\vec{S}_1 \cdot \vec{v}_2)^2 + \\ 3 \vec{S}_1 \cdot \vec{v}_1 \vec{S}_1 \cdot \vec{v}_2 + \frac{1}{2} \vec{S}_1 \cdot \vec{S}_1 \vec{v}_2 \cdot \vec{v}_2 \Big) + \frac{-12 \hat{n} \cdot \vec{S}_1 \hat{n} \cdot \vec{S}_1 \hat{n} \cdot \vec{v}_2 + 3 \hat{n} \cdot \vec{S}_1 \vec{S}_1 \cdot \vec{v}_2 + 3 \hat{n} \cdot \vec{S}_1 \vec{S}_1 \cdot \vec{v}_2}{r^4} \Big\}$$

{DiagS1CES2[3, 4, 14],

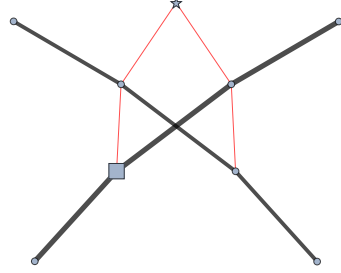

,  $G^3 m_2^2 C_{ES^2_1}$

$$\left( \frac{1}{r^5} \left( 3 (\hat{n} \cdot \vec{S}_1)^2 (\hat{n} \cdot \vec{v}_2)^2 - \frac{9}{4} (\hat{n} \cdot \vec{S}_1)^2 \hat{n} \cdot \vec{v}_1 \hat{n} \cdot \vec{v}_2 - \frac{3}{4} \vec{v}_1 \cdot \vec{v}_2 (\hat{n} \cdot \vec{S}_1)^2 + \frac{3}{2} \hat{n} \cdot \vec{S}_1 \hat{n} \cdot \vec{v}_2 \vec{S}_1 \cdot \vec{v}_1 - \frac{3}{2} \hat{n} \cdot \vec{S}_1 \hat{n} \cdot \vec{v}_2 \vec{S}_1 \cdot \vec{v}_2 - \right. \right. \\ \left. \left. \frac{1}{2} \vec{S}_1 \cdot \vec{S}_1 (\hat{n} \cdot \vec{v}_2)^2 + \frac{1}{4} \vec{S}_1 \cdot \vec{S}_1 \hat{n} \cdot \vec{v}_1 \hat{n} \cdot \vec{v}_2 + \frac{1}{4} \vec{S}_1 \cdot \vec{S}_1 \vec{v}_1 \cdot \vec{v}_2 \right) + \frac{\frac{3}{2} \hat{n} \cdot \vec{S}_1 \hat{n} \cdot \vec{S}_1 \hat{n} \cdot \vec{v}_2 - \frac{1}{2} \vec{S}_1 \cdot \vec{S}_1 \hat{n} \cdot \vec{v}_2}{r^4} \right\}$$

{DiagS1CES2[3, 4, 15],

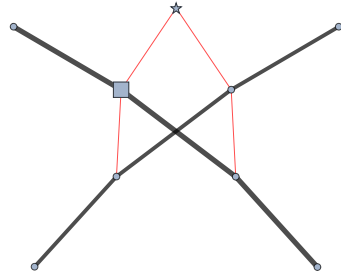

,

$$G^3 m_2^2 C_{ES^2_1} \left( \frac{1}{r^5} \left( -12 (\hat{n} \cdot \vec{S}_1)^2 (\hat{n} \cdot \vec{v}_2)^2 + 30 (\hat{n} \cdot \vec{S}_1)^2 \hat{n} \cdot \vec{v}_1 \hat{n} \cdot \vec{v}_2 - 6 \vec{v}_1 \cdot \vec{v}_2 (\hat{n} \cdot \vec{S}_1)^2 - \right. \right. \\ 12 \hat{n} \cdot \vec{S}_1 \hat{n} \cdot \vec{v}_2 \vec{S}_1 \cdot \vec{v}_1 - 9 \hat{n} \cdot \vec{S}_1 \hat{n} \cdot \vec{v}_1 \vec{S}_1 \cdot \vec{v}_2 + 9 \hat{n} \cdot \vec{S}_1 \hat{n} \cdot \vec{v}_2 \vec{S}_1 \cdot \vec{v}_2 - 2 \vec{S}_1 \cdot \vec{S}_1 (\hat{n} \cdot \vec{v}_1)^2 - \\ \vec{S}_1 \cdot \vec{S}_1 (\hat{n} \cdot \vec{v}_2)^2 + 4 \vec{S}_1 \cdot \vec{S}_1 \hat{n} \cdot \vec{v}_1 \hat{n} \cdot \vec{v}_2 - \frac{3}{2} (\vec{S}_1 \cdot \vec{v}_2)^2 + 3 \vec{S}_1 \cdot \vec{v}_1 \vec{S}_1 \cdot \vec{v}_2 + \frac{1}{2} \vec{S}_1 \cdot \vec{S}_1 \vec{v}_2 \cdot \vec{v}_2 \Big) + \\ \left. \frac{-12 \hat{n} \cdot \vec{S}_1 \hat{n} \cdot \vec{S}_1 \hat{n} \cdot \vec{v}_2 - \vec{S}_1^2 \hat{n} \cdot \vec{v}_2 + 3 \hat{n} \cdot \vec{S}_1 \vec{S}_1 \cdot \vec{v}_2 + 3 \hat{n} \cdot \vec{S}_1 \vec{S}_1 \cdot \vec{v}_2 + \vec{S}_1^2 \hat{n} \cdot \vec{v}_1}{r^4} \right\}$$

{DiagS1CES2[3, 4, 16],

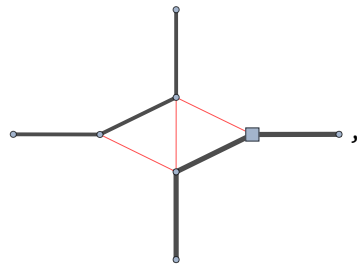

,

$$G^3 m_2^2 C_{ES^2 1} \left( \frac{\vec{S}_1 \cdot \vec{a}_1 \hat{n} \cdot \vec{S}_1 + \hat{n} \cdot \vec{S}_1 \vec{S}_1 \cdot \vec{v}_1 - 2 \vec{S}_1 \cdot \vec{S}_1 \hat{n} \cdot \vec{v}_1 + \hat{n} \cdot \vec{S}_1 \vec{S}_1 \cdot \vec{v}_1}{r^4} + \frac{1}{r^5} \left( \frac{9}{2} \vec{v}_1 \cdot \vec{v}_1 (\hat{n} \cdot \vec{S}_1)^2 + \frac{9}{2} \vec{v}_2 \cdot \vec{v}_2 (\hat{n} \cdot \vec{S}_1)^2 + \right. \right. \\ \left. \left. \frac{3}{2} \hat{n} \cdot \vec{S}_1 \hat{n} \cdot \vec{v}_1 \vec{S}_1 \cdot \vec{v}_1 - \frac{3}{2} \vec{S}_1 \cdot \vec{S}_1 (\hat{n} \cdot \vec{v}_1)^2 - \frac{1}{2} (\vec{S}_1 \cdot \vec{v}_1)^2 - \vec{S}_1 \cdot \vec{S}_1 \vec{v}_1 \cdot \vec{v}_1 - \frac{3}{2} \vec{S}_1 \cdot \vec{S}_1 \vec{v}_2 \cdot \vec{v}_2 \right) + \frac{S_1^2}{r^3} \right) \Bigg\}$$

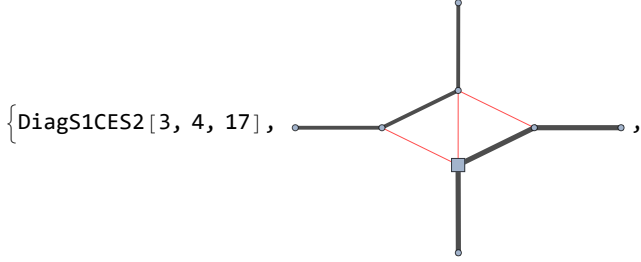

$$G^3 m_2^2 C_{ES^2 1} \left( \frac{\vec{S}_1 \cdot \vec{S}_1 \hat{n} \cdot \vec{a}_1 - 3 \vec{S}_1 \cdot \vec{S}_1 \hat{n} \cdot \vec{a}_2}{r^4} + \frac{1}{r^5} \left( -16 \vec{v}_1 \cdot \vec{v}_1 (\hat{n} \cdot \vec{S}_1)^2 + 36 \vec{v}_2 \cdot \vec{v}_2 (\hat{n} \cdot \vec{S}_1)^2 - \right. \right. \\ \left. \left. 6 \hat{n} \cdot \vec{S}_1 \hat{n} \cdot \vec{v}_1 \vec{S}_1 \cdot \vec{v}_1 + 10 \hat{n} \cdot \vec{S}_1 \hat{n} \cdot \vec{v}_2 \vec{S}_1 \cdot \vec{v}_1 - 5 \vec{S}_1 \cdot \vec{S}_1 (\hat{n} \cdot \vec{v}_1)^2 - 19 \vec{S}_1 \cdot \vec{S}_1 (\hat{n} \cdot \vec{v}_2)^2 + \right. \right. \\ \left. \left. 22 \vec{S}_1 \cdot \vec{S}_1 \hat{n} \cdot \vec{v}_1 \hat{n} \cdot \vec{v}_2 + (\vec{S}_1 \cdot \vec{v}_1)^2 - 2 \vec{S}_1 \cdot \vec{v}_1 \vec{S}_1 \cdot \vec{v}_2 + 6 \vec{S}_1 \cdot \vec{S}_1 \vec{v}_1 \cdot \vec{v}_1 - 4 \vec{S}_1 \cdot \vec{S}_1 \vec{v}_1 \cdot \vec{v}_2 - 9 \vec{S}_1 \cdot \vec{S}_1 \vec{v}_2 \cdot \vec{v}_2 \right) \right) \Bigg\}$$

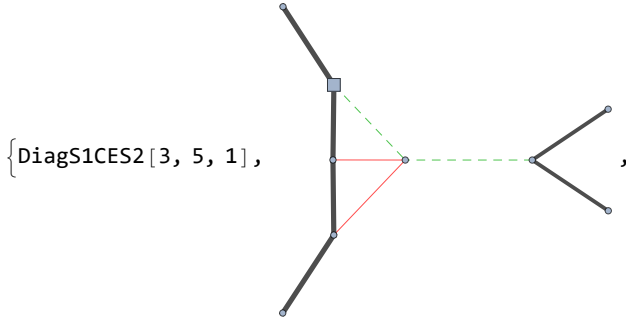

$$G^3 m_1 m_2 C_{ES^2 1} \left( \frac{-\frac{144}{7} \vec{v}_1 \cdot \vec{v}_2 (\hat{n} \cdot \vec{S}_1)^2 + \frac{96}{7} \hat{n} \cdot \vec{S}_1 \hat{n} \cdot \vec{v}_2 \vec{S}_1 \cdot \vec{v}_1 - \frac{96}{7} \hat{n} \cdot \vec{S}_1 \hat{n} \cdot \vec{v}_1 \vec{S}_1 \cdot \vec{v}_2 + \frac{48}{7} \vec{S}_1 \cdot \vec{S}_1 \vec{v}_1 \cdot \vec{v}_2}{r^5} + \right. \\ \left. \frac{\frac{48}{5} \hat{n} \cdot \vec{S}_1 \vec{S}_1 \cdot \vec{v}_2 - \frac{32}{5} \vec{S}_1 \cdot \vec{S}_1 \hat{n} \cdot \vec{v}_2 + \frac{48}{5} \hat{n} \cdot \vec{S}_1 \vec{S}_1 \cdot \vec{v}_2}{r^4} \right) \Bigg\}$$

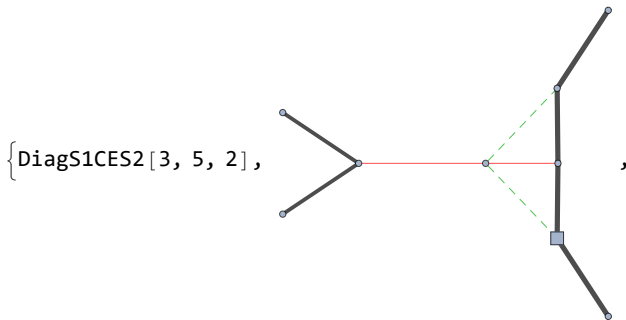

$$G^3 m_1 m_2 C_{ES^2 1} \left\{ \frac{\frac{144}{7} \vec{v}_1 \cdot \vec{v}_1 \left( \hat{n} \cdot \vec{S}_1 \right)^2 - \frac{48}{7} \vec{S}_1 \cdot \vec{S}_1 \vec{v}_1 \cdot \vec{v}_1}{r^5} + \frac{-\frac{48}{5} \hat{n} \cdot \vec{S}_1 \vec{S}_1 \cdot \vec{v}_1 + \frac{32}{5} \vec{S}_1 \cdot \vec{S}_1 \hat{n} \cdot \vec{v}_1 - \frac{48}{5} \hat{n} \cdot \vec{S}_1 \vec{S}_1 \cdot \vec{v}_1}{r^4} \right\}$$

{DiagS1CES2[3, 5, 3],

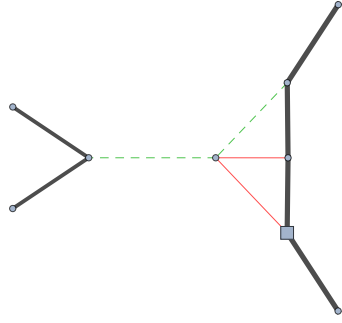

,

$$\frac{G^3 m_1 m_2 C_{ES^2 1} \left( -\frac{192}{7} \vec{v}_1 \cdot \vec{v}_2 \left( \hat{n} \cdot \vec{S}_1 \right)^2 - \frac{96}{7} \hat{n} \cdot \vec{S}_1 \hat{n} \cdot \vec{v}_2 \vec{S}_1 \cdot \vec{v}_1 + \frac{96}{7} \hat{n} \cdot \vec{S}_1 \hat{n} \cdot \vec{v}_1 \vec{S}_1 \cdot \vec{v}_2 + \frac{64}{7} \vec{S}_1 \cdot \vec{S}_1 \vec{v}_1 \cdot \vec{v}_2 \right)}{r^5}$$

{DiagS1CES2[3, 5, 4],

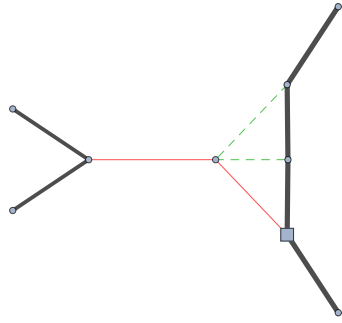

,

$$\frac{G^3 m_1 m_2 C_{ES^2 1} \left( \frac{24}{7} \vec{v}_1 \cdot \vec{v}_1 \left( \hat{n} \cdot \vec{S}_1 \right)^2 - \frac{8}{7} \vec{S}_1 \cdot \vec{S}_1 \vec{v}_1 \cdot \vec{v}_1 \right)}{r^5}$$

{DiagS1CES2[3, 5, 5],

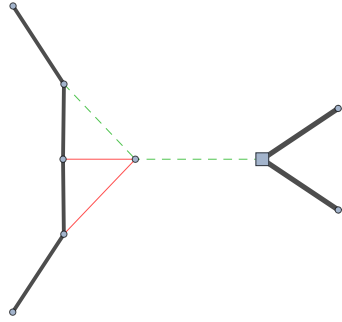

,

$$\frac{G^3 m_2^3 C_{ES^2 1} \left( \frac{48 \vec{S}_1 \cdot \vec{S}_1 \vec{v}_1 \cdot \vec{v}_2 - 80 \vec{v}_1 \cdot \vec{v}_2 \left( \hat{n} \cdot \vec{S}_1 \right)^2}{r^5} + \frac{16 \hat{n} \cdot \vec{S}_1 \vec{S}_1 \cdot \vec{v}_2 - 32 \vec{S}_1 \cdot \vec{S}_1 \hat{n} \cdot \vec{v}_2 + 16 \hat{n} \cdot \vec{S}_1 \vec{S}_1 \cdot \vec{v}_2}{r^4} \right)}{m_1}$$

{DiagS1CES2[3, 5, 6],

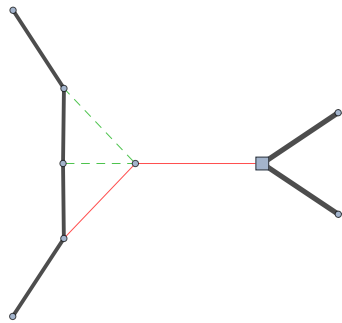

,

$$\frac{G^3 m_2^3 C_{ES^2 1} \left( 40 \vec{v}_2 \cdot \vec{v}_2 \left( \hat{n} \cdot \vec{S}_1 \right)^2 - 24 \vec{S}_1 \cdot \vec{S}_1 \vec{v}_2 \cdot \vec{v}_2 \right)}{m_1 r^5}$$



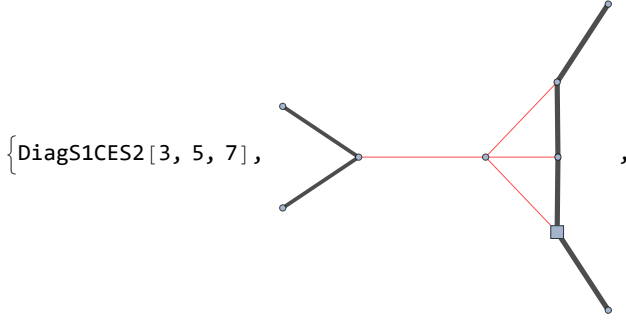

$$\begin{aligned}
 & G^3 m_1 m_2 \left( \frac{1}{r^4} \left( -\frac{404}{49} \hat{n} \cdot \vec{S}_1 \hat{n} \cdot \vec{S}_1 \hat{n} \cdot \vec{v}_1 + \frac{3476 \vec{S}_1 \cdot \vec{S}_1 \hat{n} \cdot \vec{v}_1}{1225} + 22 \hat{n} \cdot \vec{S}_1 \hat{n} \cdot \vec{S}_1 \hat{n} \cdot \vec{v}_2 + \right. \right. \\
 & \quad \left. \frac{676 \hat{n} \cdot \vec{S}_1 \vec{S}_1 \cdot \vec{v}_1}{1225} - \frac{74}{25} \hat{n} \cdot \vec{S}_1 \vec{S}_1 \cdot \vec{v}_2 - \frac{174}{25} \hat{n} \cdot \vec{v}_2 \vec{S}_1 \cdot \vec{S}_1 + \frac{676 \hat{n} \cdot \vec{S}_1 \vec{S}_1 \cdot \vec{v}_1}{1225} - \frac{74}{25} \hat{n} \cdot \vec{S}_1 \vec{S}_1 \cdot \vec{v}_2 \right) + \\
 & \quad \frac{1}{r^5} \left( \frac{61}{3} (\hat{n} \cdot \vec{v}_1)^2 (\hat{n} \cdot \vec{S}_1)^2 - 95 \hat{n} \cdot \vec{v}_1 \hat{n} \cdot \vec{v}_2 (\hat{n} \cdot \vec{S}_1)^2 - \frac{69}{49} \vec{v}_1 \cdot \vec{v}_1 (\hat{n} \cdot \vec{S}_1)^2 + 11 \vec{v}_1 \cdot \vec{v}_2 (\hat{n} \cdot \vec{S}_1)^2 - \right. \\
 & \quad \left. \frac{444}{49} \hat{n} \cdot \vec{v}_1 \vec{S}_1 \cdot \vec{v}_1 \hat{n} \cdot \vec{S}_1 + 22 \hat{n} \cdot \vec{v}_2 \vec{S}_1 \cdot \vec{v}_1 \hat{n} \cdot \vec{S}_1 + 22 \hat{n} \cdot \vec{v}_1 \vec{S}_1 \cdot \vec{v}_2 \hat{n} \cdot \vec{S}_1 + \frac{1636 (\vec{S}_1 \cdot \vec{v}_1)^2}{3675} - \right. \\
 & \quad \left. \frac{655}{147} (\hat{n} \cdot \vec{v}_1)^2 \vec{S}_1 \cdot \vec{S}_1 + 21 \hat{n} \cdot \vec{v}_1 \hat{n} \cdot \vec{v}_2 \vec{S}_1 \cdot \vec{S}_1 - \frac{74}{25} \vec{S}_1 \cdot \vec{v}_1 \vec{S}_1 \cdot \vec{v}_2 + \frac{1693 \vec{S}_1 \cdot \vec{S}_1 \vec{v}_1 \cdot \vec{v}_1}{3675} - \frac{87}{25} \vec{S}_1 \cdot \vec{S}_1 \vec{v}_1 \cdot \vec{v}_2 \right) + \\
 & \quad \left( \frac{1}{r^4} \left( \frac{72}{7} \hat{n} \cdot \vec{S}_1 \hat{n} \cdot \vec{S}_1 \hat{n} \cdot \vec{v}_1 - \frac{72}{35} \vec{S}_1 \cdot \vec{S}_1 \hat{n} \cdot \vec{v}_1 - 36 \hat{n} \cdot \vec{S}_1 \hat{n} \cdot \vec{S}_1 \hat{n} \cdot \vec{v}_2 - \frac{72}{35} \hat{n} \cdot \vec{S}_1 \vec{S}_1 \cdot \vec{v}_1 + \right. \right. \\
 & \quad \left. \frac{36}{5} \hat{n} \cdot \vec{S}_1 \vec{S}_1 \cdot \vec{v}_2 + \frac{36}{5} \hat{n} \cdot \vec{v}_2 \vec{S}_1 \cdot \vec{S}_1 - \frac{72}{35} \hat{n} \cdot \vec{S}_1 \vec{S}_1 \cdot \vec{v}_1 + \frac{36}{5} \hat{n} \cdot \vec{S}_1 \vec{S}_1 \cdot \vec{v}_2 \right) + \frac{1}{r^5} \\
 & \quad \left( -22 (\hat{n} \cdot \vec{v}_1)^2 (\hat{n} \cdot \vec{S}_1)^2 + 126 \hat{n} \cdot \vec{v}_1 \hat{n} \cdot \vec{v}_2 (\hat{n} \cdot \vec{S}_1)^2 + \frac{22}{7} \vec{v}_1 \cdot \vec{v}_1 (\hat{n} \cdot \vec{S}_1)^2 - 18 \vec{v}_1 \cdot \vec{v}_2 (\hat{n} \cdot \vec{S}_1)^2 + \right. \\
 & \quad \frac{88}{7} \hat{n} \cdot \vec{v}_1 \vec{S}_1 \cdot \vec{v}_1 \hat{n} \cdot \vec{S}_1 - 36 \hat{n} \cdot \vec{v}_2 \vec{S}_1 \cdot \vec{v}_1 \hat{n} \cdot \vec{S}_1 - 36 \hat{n} \cdot \vec{v}_1 \vec{S}_1 \cdot \vec{v}_2 \hat{n} \cdot \vec{S}_1 - \frac{44}{35} (\vec{S}_1 \cdot \vec{v}_1)^2 + \frac{22}{7} (\hat{n} \cdot \vec{v}_1)^2 \vec{S}_1 \cdot \vec{S}_1 - \\
 & \quad \left. 18 \hat{n} \cdot \vec{v}_1 \hat{n} \cdot \vec{v}_2 \vec{S}_1 \cdot \vec{S}_1 + \frac{36}{5} \vec{S}_1 \cdot \vec{v}_1 \vec{S}_1 \cdot \vec{v}_2 - \frac{22}{35} \vec{S}_1 \cdot \vec{S}_1 \vec{v}_1 \cdot \vec{v}_1 + \frac{18}{5} \vec{S}_1 \cdot \vec{S}_1 \vec{v}_1 \cdot \vec{v}_2 \right) \log \left( \frac{r}{R_\theta} \right) + \\
 & \quad \frac{1}{\epsilon_d} \left( \frac{1}{r^4} \left( -\frac{24}{7} \hat{n} \cdot \vec{S}_1 \hat{n} \cdot \vec{S}_1 \hat{n} \cdot \vec{v}_1 + \frac{24}{35} \vec{S}_1 \cdot \vec{S}_1 \hat{n} \cdot \vec{v}_1 + 12 \hat{n} \cdot \vec{S}_1 \hat{n} \cdot \vec{S}_1 \hat{n} \cdot \vec{v}_2 + \frac{24}{35} \hat{n} \cdot \vec{S}_1 \vec{S}_1 \cdot \vec{v}_1 - \right. \right. \\
 & \quad \left. \frac{12}{5} \hat{n} \cdot \vec{S}_1 \vec{S}_1 \cdot \vec{v}_2 - \frac{12}{5} \hat{n} \cdot \vec{v}_2 \vec{S}_1 \cdot \vec{S}_1 + \frac{24}{35} \hat{n} \cdot \vec{S}_1 \vec{S}_1 \cdot \vec{v}_1 - \frac{12}{5} \hat{n} \cdot \vec{S}_1 \vec{S}_1 \cdot \vec{v}_2 \right) + \frac{1}{r^5} \\
 & \quad \left( \frac{22}{3} (\hat{n} \cdot \vec{v}_1)^2 (\hat{n} \cdot \vec{S}_1)^2 - 42 \hat{n} \cdot \vec{v}_1 \hat{n} \cdot \vec{v}_2 (\hat{n} \cdot \vec{S}_1)^2 - \frac{22}{21} \vec{v}_1 \cdot \vec{v}_1 (\hat{n} \cdot \vec{S}_1)^2 + 6 \vec{v}_1 \cdot \vec{v}_2 (\hat{n} \cdot \vec{S}_1)^2 - \right. \\
 & \quad \frac{88}{21} \hat{n} \cdot \vec{v}_1 \vec{S}_1 \cdot \vec{v}_1 \hat{n} \cdot \vec{S}_1 + 12 \hat{n} \cdot \vec{v}_2 \vec{S}_1 \cdot \vec{v}_1 \hat{n} \cdot \vec{S}_1 + 12 \hat{n} \cdot \vec{v}_1 \vec{S}_1 \cdot \vec{v}_2 \hat{n} \cdot \vec{S}_1 + \frac{44}{105} (\vec{S}_1 \cdot \vec{v}_1)^2 - \frac{22}{21} (\hat{n} \cdot \vec{v}_1)^2 \vec{S}_1 \cdot \vec{S}_1 + \\
 & \quad \left. \left. 6 \hat{n} \cdot \vec{v}_1 \hat{n} \cdot \vec{v}_2 \vec{S}_1 \cdot \vec{S}_1 - \frac{12}{5} \vec{S}_1 \cdot \vec{v}_1 \vec{S}_1 \cdot \vec{v}_2 + \frac{22}{105} \vec{S}_1 \cdot \vec{S}_1 \vec{v}_1 \cdot \vec{v}_1 - \frac{6}{5} \vec{S}_1 \cdot \vec{S}_1 \vec{v}_1 \cdot \vec{v}_2 \right) \right) \Bigg) c_{\text{ES}^2_1} \}
 \end{aligned}$$

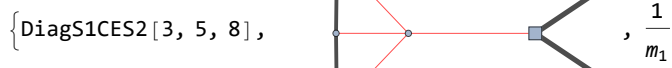

$$\frac{1}{\epsilon_d} \left( \frac{20 \hat{n} \cdot \vec{S}_1 \hat{n} \cdot \vec{S}_1 \hat{n} \cdot \vec{v}_2 - 4 \vec{S}_1 \cdot \vec{S}_1 \hat{n} \cdot \vec{v}_2 - 4 \hat{n} \cdot \vec{S}_1 \vec{S}_1 \cdot \vec{v}_2 - 4 \hat{n} \cdot \vec{S}_1 \vec{S}_1 \cdot \vec{v}_2}{r^4} + \frac{1}{r^5} \right)$$

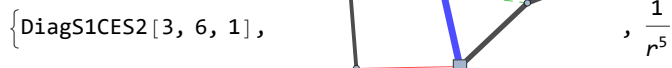

$$G^3 m_2^2 C_{E\mathbb{S}^2_1} \left\{ 44 \vec{v}_1 \cdot \vec{v}_2 \left( \hat{n} \cdot \vec{S}_1 \right)^2 - 16 \hat{n} \cdot \vec{S}_1 \hat{n} \cdot \vec{v}_2 \vec{S}_1 \cdot \vec{v}_1 - 16 \hat{n} \cdot \vec{S}_1 \hat{n} \cdot \vec{v}_1 \vec{S}_1 \cdot \vec{v}_2 + \right. \\ \left. 32 \vec{S}_1 \cdot \vec{S}_1 \hat{n} \cdot \vec{v}_1 \hat{n} \cdot \vec{v}_2 + 12 \vec{S}_1 \cdot \vec{v}_1 \vec{S}_1 \cdot \vec{v}_2 - 40 \vec{S}_1 \cdot \vec{S}_1 \vec{v}_1 \cdot \vec{v}_2 \right\} \Bigg\}$$

{DiagS1CES2[3, 6, 2],

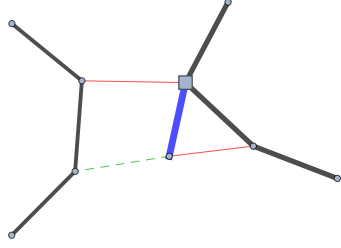

,

$$G^3 m_2^2 C_{ES^2 1} \left( \frac{14 \hat{n} \cdot \vec{a}_2 (\hat{n} \cdot \vec{S}_1)^2 + 4 \vec{S}_1 \cdot \vec{a}_2 \hat{n} \cdot \vec{S}_1 - 14 \vec{S}_1 \cdot \vec{S}_1 \hat{n} \cdot \vec{a}_2}{r^4} + \frac{1}{r^5} \left( 32 (\hat{n} \cdot \vec{S}_1)^2 (\hat{n} \cdot \vec{v}_2)^2 - \right. \right. \\ \left. \left. 32 (\hat{n} \cdot \vec{S}_1)^2 \hat{n} \cdot \vec{v}_1 \hat{n} \cdot \vec{v}_2 + 18 \hat{n} \cdot \vec{S}_1 \hat{n} \cdot \vec{v}_2 \vec{S}_1 \cdot \vec{v}_1 + 2 \hat{n} \cdot \vec{S}_1 \hat{n} \cdot \vec{v}_1 \vec{S}_1 \cdot \vec{v}_2 - 20 \hat{n} \cdot \vec{S}_1 \hat{n} \cdot \vec{v}_2 \vec{S}_1 \cdot \vec{v}_2 - \right. \right. \\ \left. \left. 4 \vec{S}_1 \cdot \vec{S}_1 (\hat{n} \cdot \vec{v}_2)^2 + 8 \vec{S}_1 \cdot \vec{S}_1 \hat{n} \cdot \vec{v}_1 \hat{n} \cdot \vec{v}_2 + 8 (\vec{S}_1 \cdot \vec{v}_2)^2 - 6 \vec{S}_1 \cdot \vec{v}_1 \vec{S}_1 \cdot \vec{v}_2 + 6 \vec{S}_1 \cdot \vec{S}_1 \vec{v}_1 \cdot \vec{v}_2 - 8 \vec{S}_1 \cdot \vec{S}_1 \vec{v}_2 \cdot \vec{v}_2 \right) \right\}$$

{DiagS1CES2[3, 6, 3],

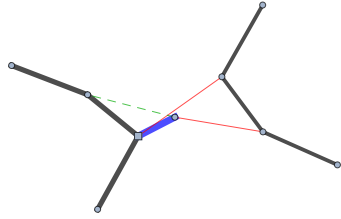

,

$$G^3 m_2^2 C_{ES^2 1} \left( \frac{-32 \hat{n} \cdot \vec{a}_1 (\hat{n} \cdot \vec{S}_1)^2 - 8 \vec{S}_1 \cdot \vec{a}_1 \hat{n} \cdot \vec{S}_1 + 32 \vec{S}_1 \cdot \vec{S}_1 \hat{n} \cdot \vec{a}_1}{r^4} + \frac{1}{r^5} \left( 32 (\hat{n} \cdot \vec{S}_1)^2 (\hat{n} \cdot \vec{v}_1)^2 - \right. \right. \\ \left. \left. 32 (\hat{n} \cdot \vec{S}_1)^2 \hat{n} \cdot \vec{v}_1 \hat{n} \cdot \vec{v}_2 - 20 \hat{n} \cdot \vec{S}_1 \hat{n} \cdot \vec{v}_1 \vec{S}_1 \cdot \vec{v}_1 + 4 \hat{n} \cdot \vec{S}_1 \hat{n} \cdot \vec{v}_2 \vec{S}_1 \cdot \vec{v}_1 + 16 \hat{n} \cdot \vec{S}_1 \hat{n} \cdot \vec{v}_1 \vec{S}_1 \cdot \vec{v}_2 - \right. \right. \\ \left. \left. 8 \vec{S}_1 \cdot \vec{S}_1 (\hat{n} \cdot \vec{v}_1)^2 + 4 \vec{S}_1 \cdot \vec{S}_1 \hat{n} \cdot \vec{v}_1 \hat{n} \cdot \vec{v}_2 + 6 (\vec{S}_1 \cdot \vec{v}_1)^2 - 8 \vec{S}_1 \cdot \vec{v}_1 \vec{S}_1 \cdot \vec{v}_2 - 6 \vec{S}_1 \cdot \vec{S}_1 \vec{v}_1 \cdot \vec{v}_1 + 8 \vec{S}_1 \cdot \vec{S}_1 \vec{v}_1 \cdot \vec{v}_2 \right) \right\}$$

{DiagS1CES2[3, 6, 4],

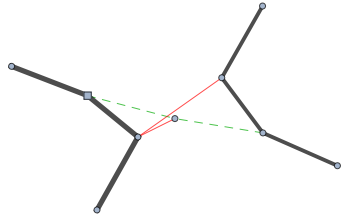

,

$$G^3 m_2^2 C_{ES^2 1} \left( \frac{-12 \vec{v}_1 \cdot \vec{v}_2 (\hat{n} \cdot \vec{S}_1)^2 + 8 \hat{n} \cdot \vec{S}_1 \hat{n} \cdot \vec{v}_2 \vec{S}_1 \cdot \vec{v}_1 - 8 \hat{n} \cdot \vec{S}_1 \hat{n} \cdot \vec{v}_1 \vec{S}_1 \cdot \vec{v}_2 + 4 \vec{S}_1 \cdot \vec{S}_1 \vec{v}_1 \cdot \vec{v}_2}{r^5} + \right. \\ \left. \frac{6 \hat{n} \cdot \vec{S}_1 \vec{S}_1 \cdot \vec{v}_2 - 4 \vec{S}_1 \cdot \vec{S}_1 \hat{n} \cdot \vec{v}_2 + 6 \hat{n} \cdot \vec{S}_1 \vec{S}_1 \cdot \vec{v}_2}{r^4} \right\}$$

{DiagS1CES2[3, 6, 5],

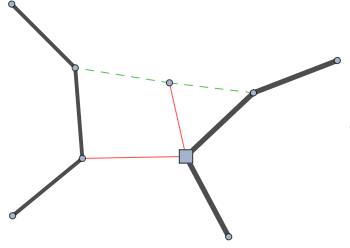

,

$$\frac{G^3 m_2^2 C_{ES^2_1} \left( -96 \vec{v}_1 \cdot \vec{v}_2 \left( \hat{n} \cdot \vec{S}_1 \right)^2 - 36 \hat{n} \cdot \vec{S}_1 \hat{n} \cdot \vec{v}_2 \vec{S}_1 \cdot \vec{v}_1 + 36 \hat{n} \cdot \vec{S}_1 \hat{n} \cdot \vec{v}_1 \vec{S}_1 \cdot \vec{v}_2 + 32 \vec{S}_1 \cdot \vec{S}_1 \vec{v}_1 \cdot \vec{v}_2 \right)}{r^5} \Bigg\}$$

{DiagS1CES2[3, 6, 6],

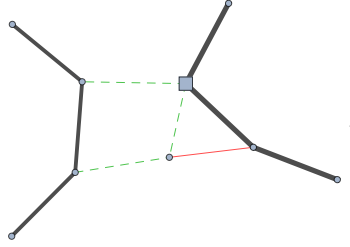

,

$$\frac{G^3 m_2^2 C_{ES^2_1} \left( 4 \vec{v}_2 \cdot \vec{v}_2 \left( \hat{n} \cdot \vec{S}_1 \right)^2 - 8 \hat{n} \cdot \vec{S}_1 \hat{n} \cdot \vec{v}_2 \vec{S}_1 \cdot \vec{v}_2 + 8 \vec{S}_1 \cdot \vec{S}_1 \left( \hat{n} \cdot \vec{v}_2 \right)^2 + 4 \left( \vec{S}_1 \cdot \vec{v}_2 \right)^2 - 8 \vec{S}_1 \cdot \vec{S}_1 \vec{v}_2 \cdot \vec{v}_2 \right)}{r^5} \Bigg\}$$

{DiagS1CES2[3, 6, 7],

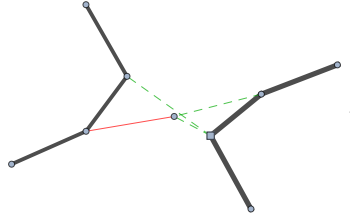

,  $\frac{1}{r^5}$

$$G^3 m_2^2 C_{ES^2_1} \left( -4 \vec{v}_1 \cdot \vec{v}_2 \left( \hat{n} \cdot \vec{S}_1 \right)^2 + 4 \hat{n} \cdot \vec{S}_1 \hat{n} \cdot \vec{v}_2 \vec{S}_1 \cdot \vec{v}_1 + 4 \hat{n} \cdot \vec{S}_1 \hat{n} \cdot \vec{v}_1 \vec{S}_1 \cdot \vec{v}_2 - 8 \vec{S}_1 \cdot \vec{S}_1 \hat{n} \cdot \vec{v}_1 \hat{n} \cdot \vec{v}_2 - 4 \vec{S}_1 \cdot \vec{v}_1 \vec{S}_1 \cdot \vec{v}_2 + 8 \vec{S}_1 \cdot \vec{S}_1 \vec{v}_1 \cdot \vec{v}_2 \right) \Bigg\}$$

{DiagS1CES2[3, 6, 8],

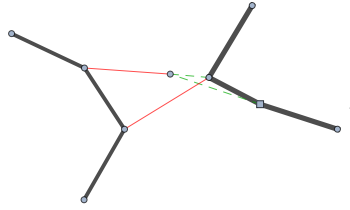

,

$$G^3 m_2^2 C_{ES^2_1} \left( \frac{12 \vec{v}_1 \cdot \vec{v}_1 \left( \hat{n} \cdot \vec{S}_1 \right)^2 - 4 \vec{S}_1 \cdot \vec{S}_1 \vec{v}_1 \cdot \vec{v}_1}{r^5} + \frac{-6 \hat{n} \cdot \vec{S}_1 \vec{S}_1 \cdot \vec{v}_1 + 4 \vec{S}_1 \cdot \vec{S}_1 \hat{n} \cdot \vec{v}_1 - 6 \hat{n} \cdot \vec{S}_1 \vec{S}_1 \cdot \vec{v}_1}{r^4} \right) \Bigg\}$$

{DiagS1CES2[3, 6, 9],

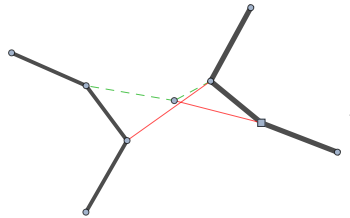

,

$$\frac{G^3 m_2^2 C_{ES^2_1} \left( -12 \vec{v}_1 \cdot \vec{v}_2 \left( \hat{n} \cdot \vec{S}_1 \right)^2 - 8 \hat{n} \cdot \vec{S}_1 \hat{n} \cdot \vec{v}_2 \vec{S}_1 \cdot \vec{v}_1 + 8 \hat{n} \cdot \vec{S}_1 \hat{n} \cdot \vec{v}_1 \vec{S}_1 \cdot \vec{v}_2 + 4 \vec{S}_1 \cdot \vec{S}_1 \vec{v}_1 \cdot \vec{v}_2 \right)}{r^5} \Bigg\}$$

$\{\text{DiagS1CES2}[3, 6, 10],$ 
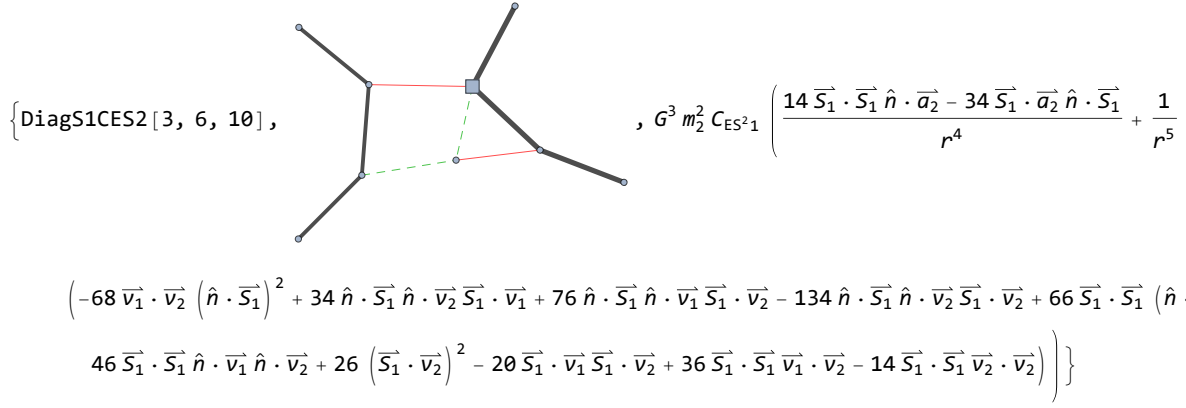
 $, G^3 m_2^2 C_{\text{ES}^2 1} \left( \frac{14 \vec{S}_1 \cdot \vec{S}_1 \hat{n} \cdot \vec{a}_2 - 34 \vec{S}_1 \cdot \vec{a}_2 \hat{n} \cdot \vec{S}_1}{r^4} + \frac{1}{r^5} \right.$ 

$$\left. \left( -68 \vec{v}_1 \cdot \vec{v}_2 (\hat{n} \cdot \vec{S}_1)^2 + 34 \hat{n} \cdot \vec{S}_1 \hat{n} \cdot \vec{v}_2 \vec{S}_1 \cdot \vec{v}_1 + 76 \hat{n} \cdot \vec{S}_1 \hat{n} \cdot \vec{v}_1 \vec{S}_1 \cdot \vec{v}_2 - 134 \hat{n} \cdot \vec{S}_1 \hat{n} \cdot \vec{v}_2 \vec{S}_1 \cdot \vec{v}_2 + 66 \vec{S}_1 \cdot \vec{S}_1 (\hat{n} \cdot \vec{v}_2)^2 - \right. \right.$$

$$\left. \left. 46 \vec{S}_1 \cdot \vec{S}_1 \hat{n} \cdot \vec{v}_1 \hat{n} \cdot \vec{v}_2 + 26 (\vec{S}_1 \cdot \vec{v}_2)^2 - 20 \vec{S}_1 \cdot \vec{v}_1 \vec{S}_1 \cdot \vec{v}_2 + 36 \vec{S}_1 \cdot \vec{S}_1 \vec{v}_1 \cdot \vec{v}_2 - 14 \vec{S}_1 \cdot \vec{S}_1 \vec{v}_2 \cdot \vec{v}_2 \right) \right\}$$

$\{\text{DiagS1CES2}[3, 6, 11],$ 
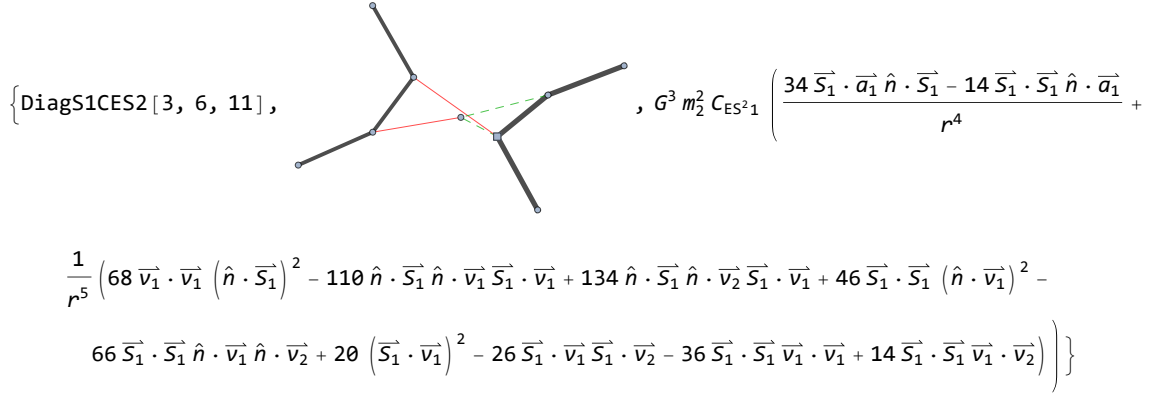
 $, G^3 m_2^2 C_{\text{ES}^2 1} \left( \frac{34 \vec{S}_1 \cdot \vec{a}_1 \hat{n} \cdot \vec{S}_1 - 14 \vec{S}_1 \cdot \vec{S}_1 \hat{n} \cdot \vec{a}_1}{r^4} + \right.$ 

$$\left. \frac{1}{r^5} \left( 68 \vec{v}_1 \cdot \vec{v}_1 (\hat{n} \cdot \vec{S}_1)^2 - 110 \hat{n} \cdot \vec{S}_1 \hat{n} \cdot \vec{v}_1 \vec{S}_1 \cdot \vec{v}_1 + 134 \hat{n} \cdot \vec{S}_1 \hat{n} \cdot \vec{v}_2 \vec{S}_1 \cdot \vec{v}_1 + 46 \vec{S}_1 \cdot \vec{S}_1 (\hat{n} \cdot \vec{v}_1)^2 - \right. \right.$$

$$\left. \left. 66 \vec{S}_1 \cdot \vec{S}_1 \hat{n} \cdot \vec{v}_1 \hat{n} \cdot \vec{v}_2 + 20 (\vec{S}_1 \cdot \vec{v}_1)^2 - 26 \vec{S}_1 \cdot \vec{v}_1 \vec{S}_1 \cdot \vec{v}_2 - 36 \vec{S}_1 \cdot \vec{S}_1 \vec{v}_1 \cdot \vec{v}_1 + 14 \vec{S}_1 \cdot \vec{S}_1 \vec{v}_1 \cdot \vec{v}_2 \right) \right\}$$

$\{\text{DiagS1CES2}[3, 6, 12],$ 
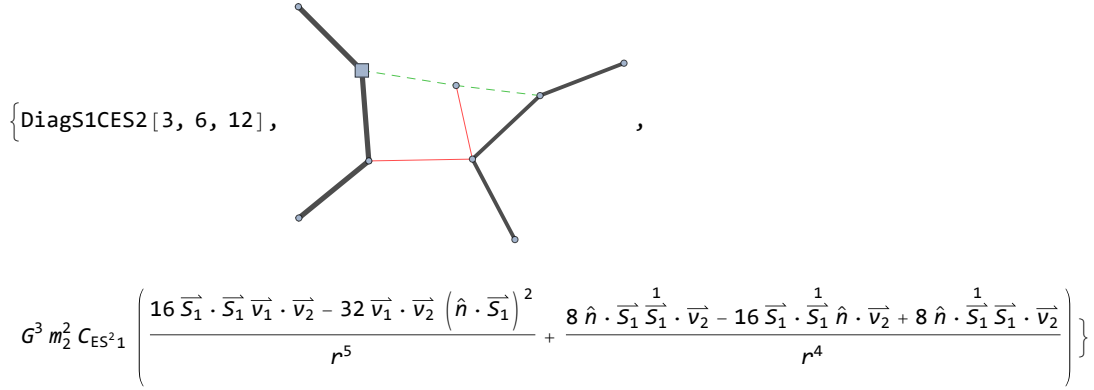
 $,$ 

$$G^3 m_2^2 C_{\text{ES}^2 1} \left\{ \frac{16 \vec{S}_1 \cdot \vec{S}_1 \vec{v}_1 \cdot \vec{v}_2 - 32 \vec{v}_1 \cdot \vec{v}_2 (\hat{n} \cdot \vec{S}_1)^2}{r^5} + \frac{8 \hat{n} \cdot \vec{S}_1 \vec{S}_1 \cdot \vec{v}_2 - 16 \vec{S}_1 \cdot \vec{S}_1 \hat{n} \cdot \vec{v}_2 + 8 \hat{n} \cdot \vec{S}_1 \vec{S}_1 \cdot \vec{v}_2}{r^4} \right\}$$

$\{\text{DiagS1CES2}[3, 6, 13],$ 
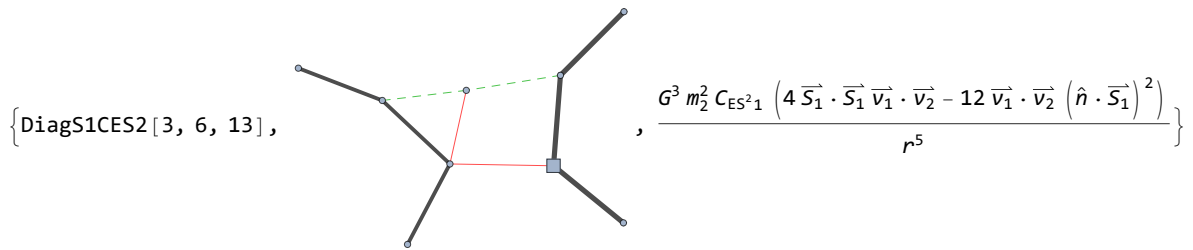
 $, \frac{G^3 m_2^2 C_{\text{ES}^2 1} \left( 4 \vec{S}_1 \cdot \vec{S}_1 \vec{v}_1 \cdot \vec{v}_2 - 12 \vec{v}_1 \cdot \vec{v}_2 (\hat{n} \cdot \vec{S}_1)^2 \right)}{r^5} \}$

$\{\text{DiagS1CES2}[3, 6, 14],$ 
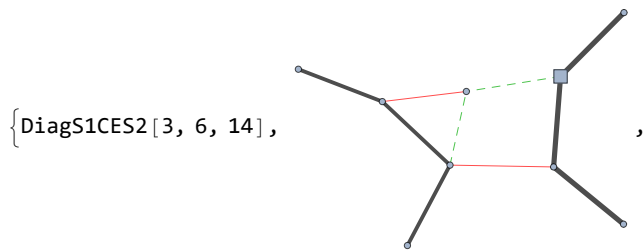
 $,$

$$G^3 m_2^2 C_{ES^2 1} \left\{ \frac{16 \vec{S}_1 \cdot \vec{S}_1 \vec{v}_1 \cdot \vec{v}_2 - 32 \vec{v}_1 \cdot \vec{v}_2 (\hat{n} \cdot \vec{S}_1)^2}{r^5} + \frac{8 \hat{n} \cdot \vec{S}_1 \vec{S}_1 \cdot \vec{v}_2 - 16 \vec{S}_1 \cdot \vec{S}_1 \hat{n} \cdot \vec{v}_2 + 8 \hat{n} \cdot \vec{S}_1 \vec{S}_1 \cdot \vec{v}_2}{r^4} \right\}$$

{DiagS1CES2[3, 6, 15], 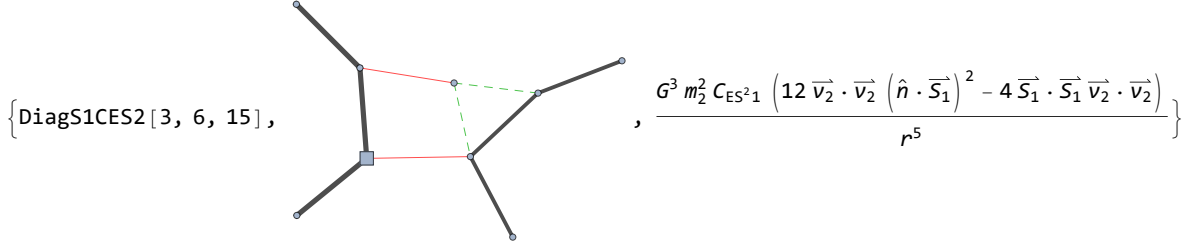 ,  $\frac{G^3 m_2^2 C_{ES^2 1} (12 \vec{v}_2 \cdot \vec{v}_2 (\hat{n} \cdot \vec{S}_1)^2 - 4 \vec{S}_1 \cdot \vec{S}_1 \vec{v}_2 \cdot \vec{v}_2)}{r^5}$  }

{DiagS1CES2[3, 6, 16], 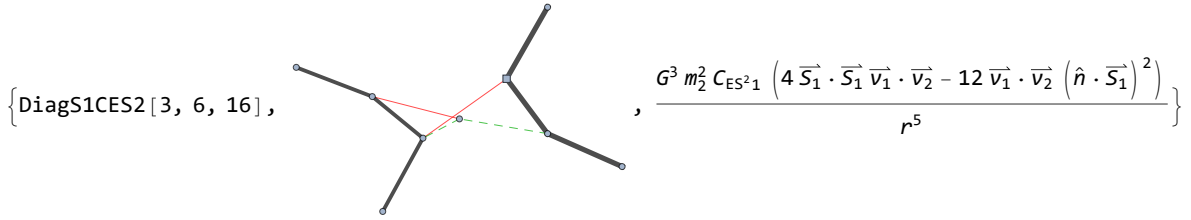 ,  $\frac{G^3 m_2^2 C_{ES^2 1} (4 \vec{S}_1 \cdot \vec{S}_1 \vec{v}_1 \cdot \vec{v}_2 - 12 \vec{v}_1 \cdot \vec{v}_2 (\hat{n} \cdot \vec{S}_1)^2)}{r^5}$  }

{DiagS1CES2[3, 6, 17], 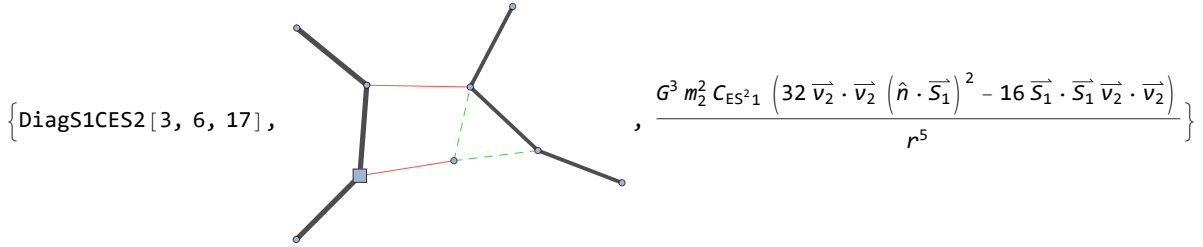 ,  $\frac{G^3 m_2^2 C_{ES^2 1} (32 \vec{v}_2 \cdot \vec{v}_2 (\hat{n} \cdot \vec{S}_1)^2 - 16 \vec{S}_1 \cdot \vec{S}_1 \vec{v}_2 \cdot \vec{v}_2)}{r^5}$  }

{DiagS1CES2[3, 6, 18], 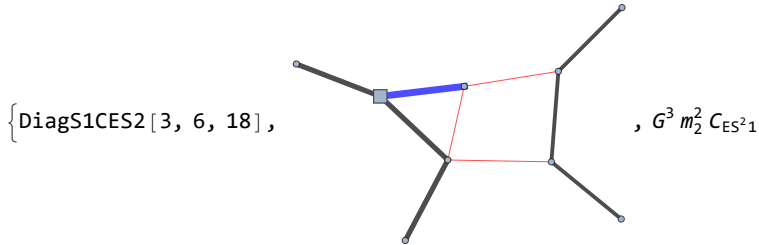 ,  $G^3 m_2^2 C_{ES^2 1}$

$$\left\{ \frac{2 \hat{n} \cdot \vec{a}_1 (\hat{n} \cdot \vec{S}_1)^2 - \vec{S}_1 \cdot \vec{a}_1 \hat{n} \cdot \vec{S}_1 + \vec{S}_1 \cdot \vec{S}_1 \hat{n} \cdot \vec{a}_1 + 8 \hat{n} \cdot \vec{S}_1 \hat{n} \cdot \vec{S}_1 \hat{n} \cdot \vec{v}_1 - \frac{5}{2} \hat{n} \cdot \vec{S}_1 \vec{S}_1 \cdot \vec{v}_1 + 3 \vec{S}_1 \cdot \vec{S}_1 \hat{n} \cdot \vec{v}_1 - \frac{5}{2} \hat{n} \cdot \vec{S}_1 \vec{S}_1 \cdot \vec{v}_1}{r^4} \right. \\ \left. + \frac{-6 (\hat{n} \cdot \vec{S}_1)^2 (\hat{n} \cdot \vec{v}_1)^2 + \vec{v}_1 \cdot \vec{v}_1 (\hat{n} \cdot \vec{S}_1)^2 + 6 \hat{n} \cdot \vec{S}_1 \hat{n} \cdot \vec{v}_1 \vec{S}_1 \cdot \vec{v}_1 - (\vec{S}_1 \cdot \vec{v}_1)^2}{r^5} + \frac{-4 (\hat{n} \cdot \vec{S}_1)^2 - 4 \hat{n} \cdot \vec{S}_1 \hat{n} \cdot \vec{S}_1}{r^3} \right\}$$

{DiagS1CES2[3, 6, 19], 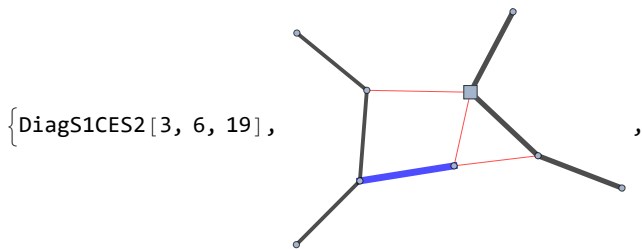 ,

$$\frac{1}{r^5} G^3 m_2^2 C_{ES^2_1} \left( \frac{87}{4} (\hat{n} \cdot \vec{S}_1)^2 (\hat{n} \cdot \vec{v}_2)^2 - \frac{45}{4} \vec{v}_2 \cdot \vec{v}_2 (\hat{n} \cdot \vec{S}_1)^2 - \right. \\ \left. 12 \hat{n} \cdot \vec{S}_1 \hat{n} \cdot \vec{v}_2 \vec{S}_1 \cdot \vec{v}_2 - \frac{13}{4} \vec{S}_1 \cdot \vec{S}_1 (\hat{n} \cdot \vec{v}_2)^2 + \frac{3}{2} (\vec{S}_1 \cdot \vec{v}_2)^2 + \frac{13}{4} \vec{S}_1 \cdot \vec{S}_1 \vec{v}_2 \cdot \vec{v}_2 \right) \Big\}$$

{DiagS1CES2[3, 6, 20],

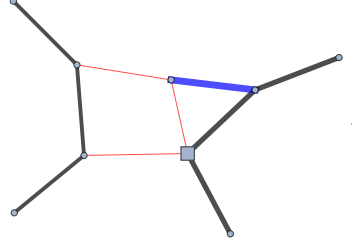

,

$$\frac{1}{r^5} G^3 m_2^2 C_{ES^2_1} \left( -144 (\hat{n} \cdot \vec{S}_1)^2 (\hat{n} \cdot \vec{v}_1)^2 + 33 \vec{v}_1 \cdot \vec{v}_1 (\hat{n} \cdot \vec{S}_1)^2 + \right. \\ \left. 69 \hat{n} \cdot \vec{S}_1 \hat{n} \cdot \vec{v}_1 \vec{S}_1 \cdot \vec{v}_1 + 25 \vec{S}_1 \cdot \vec{S}_1 (\hat{n} \cdot \vec{v}_1)^2 - 6 (\vec{S}_1 \cdot \vec{v}_1)^2 - 9 \vec{S}_1 \cdot \vec{S}_1 \vec{v}_1 \cdot \vec{v}_1 \right) \Big\}$$

{DiagS1CES2[3, 6, 21],

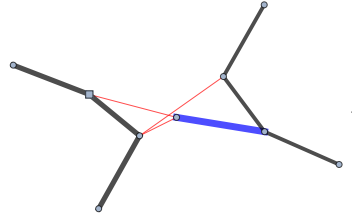

,  $\frac{1}{r^5}$

$$G^3 m_2^2 C_{ES^2_1} \left( \frac{15}{4} (\hat{n} \cdot \vec{S}_1)^2 (\hat{n} \cdot \vec{v}_2)^2 - \frac{5}{4} \vec{v}_2 \cdot \vec{v}_2 (\hat{n} \cdot \vec{S}_1)^2 - 3 \hat{n} \cdot \vec{S}_1 \hat{n} \cdot \vec{v}_2 \vec{S}_1 \cdot \vec{v}_2 - \right. \\ \left. \frac{1}{4} \vec{S}_1 \cdot \vec{S}_1 (\hat{n} \cdot \vec{v}_2)^2 + \frac{1}{2} (\vec{S}_1 \cdot \vec{v}_2)^2 + \frac{1}{4} \vec{S}_1 \cdot \vec{S}_1 \vec{v}_2 \cdot \vec{v}_2 \right) \Big\}$$

{DiagS1CES2[3, 6, 22],

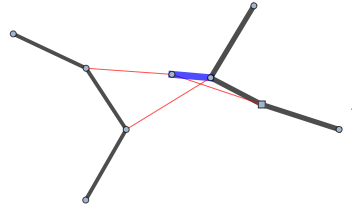

,  $\frac{1}{r^5}$

$$G^3 m_2^2 C_{ES^2_1} \left( 90 (\hat{n} \cdot \vec{S}_1)^2 (\hat{n} \cdot \vec{v}_1)^2 - 15 \vec{v}_1 \cdot \vec{v}_1 (\hat{n} \cdot \vec{S}_1)^2 - 54 \hat{n} \cdot \vec{S}_1 \hat{n} \cdot \vec{v}_1 \vec{S}_1 \cdot \vec{v}_1 - \right. \\ \left. 12 \vec{S}_1 \cdot \vec{S}_1 (\hat{n} \cdot \vec{v}_1)^2 + 6 (\vec{S}_1 \cdot \vec{v}_1)^2 + 3 \vec{S}_1 \cdot \vec{S}_1 \vec{v}_1 \cdot \vec{v}_1 \right) \Big\}$$

{DiagS1CES2[3, 6, 23],

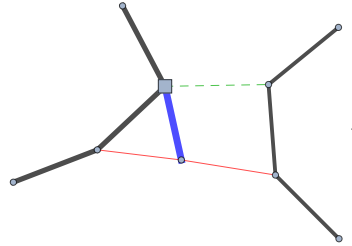

,

$$G^3 m_2^2 C_{ES^2_1} \left( \frac{16 \hat{n} \cdot \vec{a}_2 (\hat{n} \cdot \vec{S}_1)^2 - 4 \vec{S}_1 \cdot \vec{a}_2 \hat{n} \cdot \vec{S}_1 - 4 \vec{S}_1 \cdot \vec{S}_1 \hat{n} \cdot \vec{a}_2}{r^4} + \frac{1}{r^5} \right. \\ \left. (5 \vec{v}_1 \cdot \vec{v}_2 (\hat{n} \cdot \vec{S}_1)^2 + 8 \vec{v}_2 \cdot \vec{v}_2 (\hat{n} \cdot \vec{S}_1)^2 - \hat{n} \cdot \vec{S}_1 \hat{n} \cdot \vec{v}_2 \vec{S}_1 \cdot \vec{v}_1 - 13 \hat{n} \cdot \vec{S}_1 \hat{n} \cdot \vec{v}_1 \vec{S}_1 \cdot \vec{v}_2 + 12 \hat{n} \cdot \vec{S}_1 \hat{n} \cdot \vec{v}_2 \vec{S}_1 \cdot \vec{v}_2 - \right.$$

$$4 \vec{S}_1 \cdot \vec{S}_1 (\hat{n} \cdot \vec{v}_2)^2 + 6 \vec{S}_1 \cdot \vec{S}_1 \hat{n} \cdot \vec{v}_1 \hat{n} \cdot \vec{v}_2 + \vec{S}_1 \cdot \vec{v}_1 \vec{S}_1 \cdot \vec{v}_2 - 14 \vec{S}_1 \cdot \vec{S}_1 \vec{v}_1 \cdot \vec{v}_2 - 8 \vec{S}_1 \cdot \vec{S}_1 \vec{v}_2 \cdot \vec{v}_2 \Bigg) \Bigg\}$$

{DiagS1CES2[3, 6, 24],

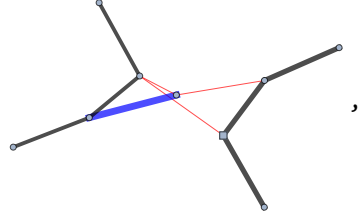

$$\frac{G^3 m_2^2 C_{ES^2_1} \left( -6 (\hat{n} \cdot \vec{S}_1)^2 (\hat{n} \cdot \vec{v}_2)^2 + 3 \vec{v}_2 \cdot \vec{v}_2 (\hat{n} \cdot \vec{S}_1)^2 + 2 \vec{S}_1 \cdot \vec{S}_1 (\hat{n} \cdot \vec{v}_2)^2 - \vec{S}_1 \cdot \vec{S}_1 \vec{v}_2 \cdot \vec{v}_2 \right)}{r^5} \Bigg\}$$

{DiagS1CES2[3, 6, 25],

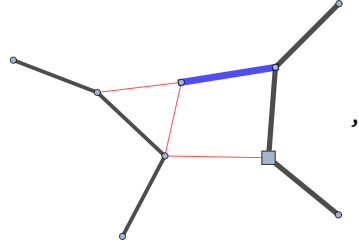

$$\frac{G^3 m_2^2 C_{ES^2_1} \left( \frac{3}{2} (\hat{n} \cdot \vec{S}_1)^2 (\hat{n} \cdot \vec{v}_1)^2 - \frac{3}{2} \vec{v}_1 \cdot \vec{v}_1 (\hat{n} \cdot \vec{S}_1)^2 - \frac{1}{2} \vec{S}_1 \cdot \vec{S}_1 (\hat{n} \cdot \vec{v}_1)^2 + \frac{1}{2} \vec{S}_1 \cdot \vec{S}_1 \vec{v}_1 \cdot \vec{v}_1 \right)}{r^5} \Bigg\}$$

{DiagS1CES2[3, 6, 26],

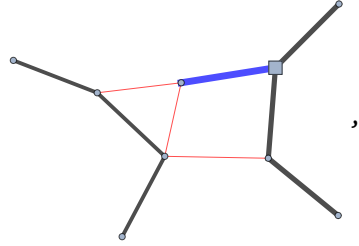

$$G^3 m_2^2 C_{ES^2_1} \left\{ \frac{-2 \hat{n} \cdot \vec{a}_1 (\hat{n} \cdot \vec{S}_1)^2 + 2 \vec{S}_1 \cdot \vec{a}_1 \hat{n} \cdot \vec{S}_1 - 8 \hat{n} \cdot \vec{S}_1 \hat{n} \cdot \vec{S}_1 \hat{n} \cdot \vec{v}_1 + 3 \hat{n} \cdot \vec{S}_1 \vec{S}_1 \cdot \vec{v}_1 - 2 \vec{S}_1 \cdot \vec{S}_1 \hat{n} \cdot \vec{v}_1 + 3 \hat{n} \cdot \vec{S}_1 \vec{S}_1 \cdot \vec{v}_1}{r^4} + \right.$$

$$\frac{12 (\hat{n} \cdot \vec{S}_1)^2 (\hat{n} \cdot \vec{v}_1)^2 - 4 \vec{v}_1 \cdot \vec{v}_1 (\hat{n} \cdot \vec{S}_1)^2 - 8 \hat{n} \cdot \vec{S}_1 \hat{n} \cdot \vec{v}_1 \vec{S}_1 \cdot \vec{v}_1 + (\vec{S}_1 \cdot \vec{v}_1)^2 + \vec{S}_1 \cdot \vec{S}_1 \vec{v}_1 \cdot \vec{v}_1}{r^5} +$$

$$\left. \frac{\left( \hat{n} \cdot \vec{S}_1 \right)^2 + \hat{n} \cdot \vec{S}_1 \hat{n} \cdot \vec{S}_1 + \vec{S}_1 \cdot \vec{S}_1 + \vec{S}_1 \cdot \vec{S}_1}{r^3} \right\}$$

{DiagS1CES2[3, 6, 27],

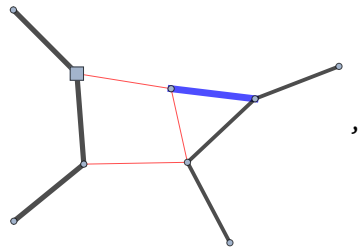



$$\frac{G^3 m_2^2 C_{ES^2 1} \left( -48 \left( \hat{n} \cdot \vec{S}_1 \right)^2 \left( \hat{n} \cdot \vec{v}_2 \right)^2 + 8 \vec{v}_2 \cdot \vec{v}_2 \left( \hat{n} \cdot \vec{S}_1 \right)^2 + 32 \hat{n} \cdot \vec{S}_1 \hat{n} \cdot \vec{v}_2 \vec{S}_1 \cdot \vec{v}_2 - 4 \left( \vec{S}_1 \cdot \vec{v}_2 \right)^2 \right)}{r^5}$$

{DiagS1CES2[3, 6, 28],

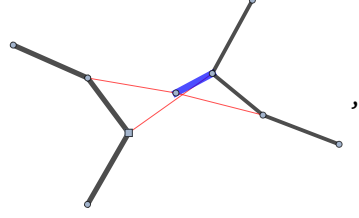

$$\frac{G^3 m_2^2 C_{ES^2 1} \left( 18 \left( \hat{n} \cdot \vec{S}_1 \right)^2 \left( \hat{n} \cdot \vec{v}_2 \right)^2 - 9 \vec{v}_2 \cdot \vec{v}_2 \left( \hat{n} \cdot \vec{S}_1 \right)^2 - 6 \vec{S}_1 \cdot \vec{S}_1 \left( \hat{n} \cdot \vec{v}_2 \right)^2 + 3 \vec{S}_1 \cdot \vec{S}_1 \vec{v}_2 \cdot \vec{v}_2 \right)}{r^5}$$

{DiagS1CES2[3, 6, 29],

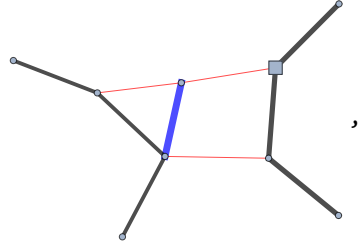

$$\frac{G^3 m_2^2 C_{ES^2 1} \left( 144 \left( \hat{n} \cdot \vec{S}_1 \right)^2 \left( \hat{n} \cdot \vec{v}_2 \right)^2 - 24 \vec{v}_2 \cdot \vec{v}_2 \left( \hat{n} \cdot \vec{S}_1 \right)^2 - 96 \hat{n} \cdot \vec{S}_1 \hat{n} \cdot \vec{v}_2 \vec{S}_1 \cdot \vec{v}_2 + 12 \left( \vec{S}_1 \cdot \vec{v}_2 \right)^2 \right)}{r^5}$$

{DiagS1CES2[3, 6, 30],

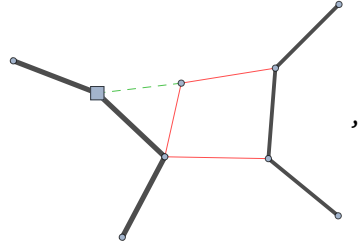

$$\frac{G^3 m_2^2 C_{ES^2 1} \left( \frac{1}{r^5} \left( 12 \left( \hat{n} \cdot \vec{S}_1 \right)^2 \left( \hat{n} \cdot \vec{v}_1 \right)^2 - \vec{v}_1 \cdot \vec{v}_1 \left( \hat{n} \cdot \vec{S}_1 \right)^2 - \vec{v}_1 \cdot \vec{v}_2 \left( \hat{n} \cdot \vec{S}_1 \right)^2 - 9 \hat{n} \cdot \vec{S}_1 \hat{n} \cdot \vec{v}_1 \vec{S}_1 \cdot \vec{v}_1 - \hat{n} \cdot \vec{S}_1 \hat{n} \cdot \vec{v}_2 \vec{S}_1 \cdot \vec{v}_1 - \right. \right. \\ \left. \left. 2 \hat{n} \cdot \vec{S}_1 \hat{n} \cdot \vec{v}_1 \vec{S}_1 \cdot \vec{v}_2 - \vec{S}_1 \cdot \vec{S}_1 \left( \hat{n} \cdot \vec{v}_1 \right)^2 + \vec{S}_1 \cdot \vec{S}_1 \hat{n} \cdot \vec{v}_1 \hat{n} \cdot \vec{v}_2 + \left( \vec{S}_1 \cdot \vec{v}_1 \right)^2 + \vec{S}_1 \cdot \vec{v}_1 \vec{S}_1 \cdot \vec{v}_2 \right) + \right. \\ \left. - 8 \hat{n} \cdot \vec{S}_1 \hat{n} \cdot \vec{S}_1 \hat{n} \cdot \vec{v}_1 - \vec{S}_1 \cdot \vec{S}_1 \hat{n} \cdot \vec{v}_1 + \frac{3}{2} \hat{n} \cdot \vec{S}_1 \vec{S}_1 \cdot \vec{v}_1 + \hat{n} \cdot \vec{S}_1 \vec{S}_1 \cdot \vec{v}_2 - 2 \vec{S}_1 \cdot \vec{S}_1 \hat{n} \cdot \vec{v}_2 + \frac{3}{2} \hat{n} \cdot \vec{S}_1 \vec{S}_1 \cdot \vec{v}_1 + \hat{n} \cdot \vec{S}_1 \vec{S}_1 \cdot \vec{v}_2 \right) \right)}{r^4}$$

{DiagS1CES2[3, 6, 31],

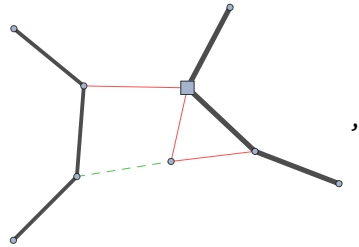

$$G^3 m_2^2 C_{ES^2 1} \left( \frac{1}{r^5} \left( 57 \left( \hat{n} \cdot \vec{S}_1 \right)^2 \left( \hat{n} \cdot \vec{v}_2 \right)^2 - \frac{201}{2} \left( \hat{n} \cdot \vec{S}_1 \right)^2 \hat{n} \cdot \vec{v}_1 \hat{n} \cdot \vec{v}_2 + \frac{45}{2} \vec{v}_1 \cdot \vec{v}_2 \left( \hat{n} \cdot \vec{S}_1 \right)^2 + \right. \right.$$

$$\left. \begin{aligned} & 33 \hat{n} \cdot \vec{S}_1 \hat{n} \cdot \vec{v}_2 \vec{S}_1 \cdot \vec{v}_1 + 24 \hat{n} \cdot \vec{S}_1 \hat{n} \cdot \vec{v}_1 \vec{S}_1 \cdot \vec{v}_2 - 33 \hat{n} \cdot \vec{S}_1 \hat{n} \cdot \vec{v}_2 \vec{S}_1 \cdot \vec{v}_2 - 8 \vec{S}_1 \cdot \vec{S}_1 (\hat{n} \cdot \vec{v}_2)^2 + \\ & \frac{29}{2} \vec{S}_1 \cdot \vec{S}_1 \hat{n} \cdot \vec{v}_1 \hat{n} \cdot \vec{v}_2 + 3 (\vec{S}_1 \cdot \vec{v}_2)^2 - 6 \vec{S}_1 \cdot \vec{v}_1 \vec{S}_1 \cdot \vec{v}_2 - \frac{11}{2} \vec{S}_1 \cdot \vec{S}_1 \vec{v}_1 \cdot \vec{v}_2 - \vec{S}_1 \cdot \vec{S}_1 \vec{v}_2 \cdot \vec{v}_2 + \\ & \frac{30 \hat{n} \cdot \vec{S}_1 \hat{n} \cdot \vec{S}_1 \hat{n} \cdot \vec{v}_2 - 6 \vec{S}_1 \cdot \vec{S}_1 \hat{n} \cdot \vec{v}_2 - 6 \hat{n} \cdot \vec{S}_1 \vec{S}_1 \cdot \vec{v}_2 - 6 \hat{n} \cdot \vec{S}_1 \vec{S}_1 \cdot \vec{v}_2}{r^4} \end{aligned} \right\}$$

{DiagS1CES2[3, 6, 32],

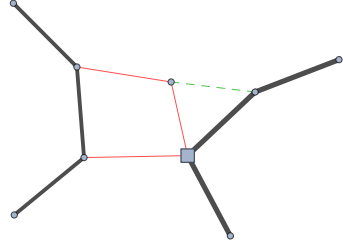

,

$$\left. \begin{aligned} & G^3 m_2^2 C_{ES^2 1} \left( \frac{1}{r^5} \left( 288 (\hat{n} \cdot \vec{S}_1)^2 (\hat{n} \cdot \vec{v}_1)^2 - 33 \vec{v}_1 \cdot \vec{v}_1 (\hat{n} \cdot \vec{S}_1)^2 - \right. \right. \\ & 33 \vec{v}_1 \cdot \vec{v}_2 (\hat{n} \cdot \vec{S}_1)^2 - 144 \hat{n} \cdot \vec{S}_1 \hat{n} \cdot \vec{v}_1 \vec{S}_1 \cdot \vec{v}_1 - 3 \hat{n} \cdot \vec{S}_1 \hat{n} \cdot \vec{v}_2 \vec{S}_1 \cdot \vec{v}_1 + 9 \hat{n} \cdot \vec{S}_1 \hat{n} \cdot \vec{v}_1 \vec{S}_1 \cdot \vec{v}_2 - \\ & 48 \vec{S}_1 \cdot \vec{S}_1 (\hat{n} \cdot \vec{v}_1)^2 - 2 \vec{S}_1 \cdot \vec{S}_1 \hat{n} \cdot \vec{v}_1 \hat{n} \cdot \vec{v}_2 + 12 (\vec{S}_1 \cdot \vec{v}_1)^2 + 7 \vec{S}_1 \cdot \vec{S}_1 \vec{v}_1 \cdot \vec{v}_1 + 11 \vec{S}_1 \cdot \vec{S}_1 \vec{v}_1 \cdot \vec{v}_2 \Big) + \\ & \left. \frac{-96 \hat{n} \cdot \vec{S}_1 \hat{n} \cdot \vec{S}_1 \hat{n} \cdot \vec{v}_1 + 30 \vec{S}_1 \cdot \vec{S}_1 \hat{n} \cdot \vec{v}_1 - 4 \vec{S}_1^2 \hat{n} \cdot \vec{v}_1 + 15 \hat{n} \cdot \vec{S}_1 \vec{S}_1 \cdot \vec{v}_1 + 15 \hat{n} \cdot \vec{S}_1 \vec{S}_1 \cdot \vec{v}_1}{r^4} \right) \end{aligned} \right\}$$

{DiagS1CES2[3, 6, 33],

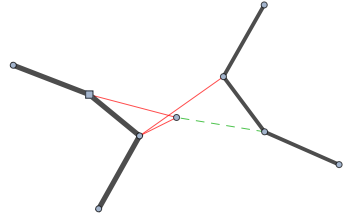

,

$$\left. \begin{aligned} & G^3 m_2^2 C_{ES^2 1} \left( \frac{1}{r^5} \left( 5 (\hat{n} \cdot \vec{S}_1)^2 (\hat{n} \cdot \vec{v}_2)^2 - \frac{25}{2} (\hat{n} \cdot \vec{S}_1)^2 \hat{n} \cdot \vec{v}_1 \hat{n} \cdot \vec{v}_2 + \frac{5}{2} \vec{v}_1 \cdot \vec{v}_2 (\hat{n} \cdot \vec{S}_1)^2 + 3 \hat{n} \cdot \vec{S}_1 \hat{n} \cdot \vec{v}_2 \vec{S}_1 \cdot \vec{v}_1 + \right. \right. \\ & 5 \hat{n} \cdot \vec{S}_1 \hat{n} \cdot \vec{v}_1 \vec{S}_1 \cdot \vec{v}_2 - 2 \hat{n} \cdot \vec{S}_1 \hat{n} \cdot \vec{v}_2 \vec{S}_1 \cdot \vec{v}_2 - \vec{S}_1 \cdot \vec{S}_1 (\hat{n} \cdot \vec{v}_2)^2 + \frac{3}{2} \vec{S}_1 \cdot \vec{S}_1 \hat{n} \cdot \vec{v}_1 \hat{n} \cdot \vec{v}_2 - \\ & \left. \left. \vec{S}_1 \cdot \vec{v}_1 \vec{S}_1 \cdot \vec{v}_2 - \frac{1}{2} \vec{S}_1 \cdot \vec{S}_1 \vec{v}_1 \cdot \vec{v}_2 \right) + \frac{2 \hat{n} \cdot \vec{S}_1 \hat{n} \cdot \vec{S}_1 \hat{n} \cdot \vec{v}_2 - \hat{n} \cdot \vec{S}_1 \vec{S}_1 \cdot \vec{v}_2 - \hat{n} \cdot \vec{S}_1 \vec{S}_1 \cdot \vec{v}_2}{r^4} \right) \end{aligned} \right\}$$

{DiagS1CES2[3, 6, 34],

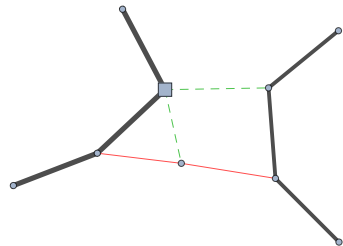

,  $\frac{1}{r^5} G^3 m_2^2 C_{ES^2 1}$

$$\left( -(\vec{v}_1 \cdot \vec{v}_2) (\hat{n} \cdot \vec{S}_1)^2 + \hat{n} \cdot \vec{S}_1 \hat{n} \cdot \vec{v}_2 \vec{S}_1 \cdot \vec{v}_1 + \hat{n} \cdot \vec{S}_1 \hat{n} \cdot \vec{v}_1 \vec{S}_1 \cdot \vec{v}_2 - 2 \vec{S}_1 \cdot \vec{S}_1 \hat{n} \cdot \vec{v}_1 \hat{n} \cdot \vec{v}_2 - \vec{S}_1 \cdot \vec{v}_1 \vec{S}_1 \cdot \vec{v}_2 + 2 \vec{S}_1 \cdot \vec{S}_1 \vec{v}_1 \cdot \vec{v}_2 \right) \Big\}$$

{DiagS1CES2[3, 6, 35],

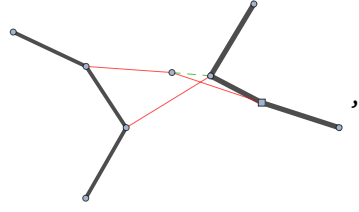

$$G^3 m_2^2 C_{ES^2 1} \left( \frac{1}{r^5} \left( 30 \left( \hat{n} \cdot \vec{S}_1 \right)^2 \left( \hat{n} \cdot \vec{v}_1 \right)^2 + 30 \left( \hat{n} \cdot \vec{S}_1 \right)^2 \hat{n} \cdot \vec{v}_1 \hat{n} \cdot \vec{v}_2 - 5 \vec{v}_1 \cdot \vec{v}_1 \left( \hat{n} \cdot \vec{S}_1 \right)^2 - 5 \vec{v}_1 \cdot \vec{v}_2 \left( \hat{n} \cdot \vec{S}_1 \right)^2 - \right. \right. \\ \left. \left. 18 \hat{n} \cdot \vec{S}_1 \hat{n} \cdot \vec{v}_1 \vec{S}_1 \cdot \vec{v}_1 - 8 \hat{n} \cdot \vec{S}_1 \hat{n} \cdot \vec{v}_2 \vec{S}_1 \cdot \vec{v}_1 - 10 \hat{n} \cdot \vec{S}_1 \hat{n} \cdot \vec{v}_1 \vec{S}_1 \cdot \vec{v}_2 - 4 \vec{S}_1 \cdot \vec{S}_1 \left( \hat{n} \cdot \vec{v}_1 \right)^2 - \right. \right. \\ \left. \left. 4 \vec{S}_1 \cdot \vec{S}_1 \hat{n} \cdot \vec{v}_1 \hat{n} \cdot \vec{v}_2 + 2 \left( \vec{S}_1 \cdot \vec{v}_1 \right)^2 + 2 \vec{S}_1 \cdot \vec{v}_1 \vec{S}_1 \cdot \vec{v}_2 + \vec{S}_1 \cdot \vec{S}_1 \vec{v}_1 \cdot \vec{v}_1 + \vec{S}_1 \cdot \vec{S}_1 \vec{v}_1 \cdot \vec{v}_2 \right) + \right. \\ \left. \left. \frac{-12 \hat{n} \cdot \vec{S}_1 \hat{n} \cdot \vec{S}_1 \hat{n} \cdot \vec{v}_1 + 2 \vec{S}_1 \cdot \vec{S}_1 \hat{n} \cdot \vec{v}_1 + 3 \hat{n} \cdot \vec{S}_1 \vec{S}_1 \cdot \vec{v}_1 + 3 \hat{n} \cdot \vec{S}_1 \vec{S}_1 \cdot \vec{v}_1}{r^4} \right) \right\}$$

{DiagS1CES2[3, 6, 36],

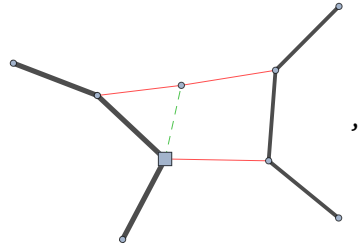

$$G^3 m_2^2 C_{ES^2 1} \left( \frac{14 \hat{n} \cdot \vec{a}_1 \left( \hat{n} \cdot \vec{S}_1 \right)^2 + 14 \hat{n} \cdot \vec{a}_2 \left( \hat{n} \cdot \vec{S}_1 \right)^2 - \frac{17}{2} \vec{S}_1 \cdot \vec{a}_1 \hat{n} \cdot \vec{S}_1 - 7 \vec{S}_1 \cdot \vec{a}_2 \hat{n} \cdot \vec{S}_1 - \frac{1}{2} \vec{S}_1 \cdot \vec{S}_1 \hat{n} \cdot \vec{a}_1 + \vec{S}_1 \cdot \vec{S}_1 \hat{n} \cdot \vec{a}_2}{r^4} + \right. \\ \left. \frac{1}{r^5} \left( -36 \left( \hat{n} \cdot \vec{S}_1 \right)^2 \left( \hat{n} \cdot \vec{v}_1 \right)^2 + 82 \left( \hat{n} \cdot \vec{S}_1 \right)^2 \left( \hat{n} \cdot \vec{v}_2 \right)^2 + 46 \left( \hat{n} \cdot \vec{S}_1 \right)^2 \hat{n} \cdot \vec{v}_1 \hat{n} \cdot \vec{v}_2 + 7 \vec{v}_1 \cdot \vec{v}_1 \left( \hat{n} \cdot \vec{S}_1 \right)^2 - \right. \right. \\ \left. \left. 8 \vec{v}_1 \cdot \vec{v}_2 \left( \hat{n} \cdot \vec{S}_1 \right)^2 - 14 \vec{v}_2 \cdot \vec{v}_2 \left( \hat{n} \cdot \vec{S}_1 \right)^2 + \frac{41}{2} \hat{n} \cdot \vec{S}_1 \hat{n} \cdot \vec{v}_1 \vec{S}_1 \cdot \vec{v}_1 - \frac{59}{2} \hat{n} \cdot \vec{S}_1 \hat{n} \cdot \vec{v}_2 \vec{S}_1 \cdot \vec{v}_1 - \right. \right. \\ \left. \left. 12 \hat{n} \cdot \vec{S}_1 \hat{n} \cdot \vec{v}_1 \vec{S}_1 \cdot \vec{v}_2 - 51 \hat{n} \cdot \vec{S}_1 \hat{n} \cdot \vec{v}_2 \vec{S}_1 \cdot \vec{v}_2 + \frac{1}{2} \vec{S}_1 \cdot \vec{S}_1 \left( \hat{n} \cdot \vec{v}_1 \right)^2 + 3 \vec{S}_1 \cdot \vec{S}_1 \left( \hat{n} \cdot \vec{v}_2 \right)^2 - \frac{21}{2} \vec{S}_1 \cdot \vec{S}_1 \hat{n} \cdot \vec{v}_1 \hat{n} \cdot \vec{v}_2 - \right. \right. \\ \left. \left. \left( \vec{S}_1 \cdot \vec{v}_1 \right)^2 + 5 \left( \vec{S}_1 \cdot \vec{v}_2 \right)^2 + \frac{13}{2} \vec{S}_1 \cdot \vec{v}_1 \vec{S}_1 \cdot \vec{v}_2 - 2 \vec{S}_1 \cdot \vec{S}_1 \vec{v}_1 \cdot \vec{v}_1 + \frac{3}{2} \vec{S}_1 \cdot \vec{S}_1 \vec{v}_1 \cdot \vec{v}_2 - \vec{S}_1 \cdot \vec{S}_1 \vec{v}_2 \cdot \vec{v}_2 \right) \right) \right\}$$

{DiagS1CES2[3, 6, 37],

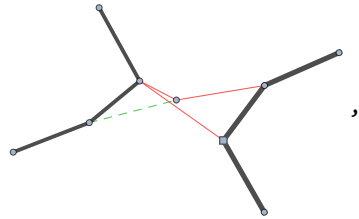

$$G^3 m_2^2 C_{ES^2 1} \left( \frac{1}{r^5} \left( 36 \left( \hat{n} \cdot \vec{S}_1 \right)^2 \left( \hat{n} \cdot \vec{v}_2 \right)^2 - 24 \left( \hat{n} \cdot \vec{S}_1 \right)^2 \hat{n} \cdot \vec{v}_1 \hat{n} \cdot \vec{v}_2 - 3 \vec{v}_1 \cdot \vec{v}_2 \left( \hat{n} \cdot \vec{S}_1 \right)^2 - \right. \right. \\ \left. \left. 3 \vec{v}_2 \cdot \vec{v}_2 \left( \hat{n} \cdot \vec{S}_1 \right)^2 + 12 \hat{n} \cdot \vec{S}_1 \hat{n} \cdot \vec{v}_2 \vec{S}_1 \cdot \vec{v}_1 - 12 \hat{n} \cdot \vec{S}_1 \hat{n} \cdot \vec{v}_2 \vec{S}_1 \cdot \vec{v}_2 - 8 \vec{S}_1 \cdot \vec{S}_1 \left( \hat{n} \cdot \vec{v}_2 \right)^2 + \right. \right. \\ \left. \left. 4 \vec{S}_1 \cdot \vec{S}_1 \hat{n} \cdot \vec{v}_1 \hat{n} \cdot \vec{v}_2 + \vec{S}_1 \cdot \vec{S}_1 \vec{v}_1 \cdot \vec{v}_2 + \vec{S}_1 \cdot \vec{S}_1 \vec{v}_2 \cdot \vec{v}_2 \right) + \frac{12 \hat{n} \cdot \vec{S}_1 \hat{n} \cdot \vec{S}_1 \hat{n} \cdot \vec{v}_2 - 4 \vec{S}_1 \cdot \vec{S}_1 \hat{n} \cdot \vec{v}_2}{r^4} \right) \right\}$$

{DiagS1CES2[3, 6, 38],

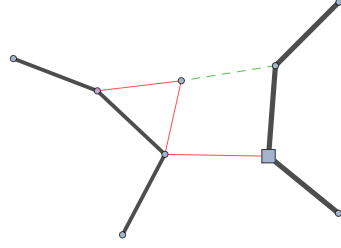

,  $G^3 m_2^2 C_{ES^2_1}$

$$\left\{ \frac{1}{r^5} \left( 15 \left( \hat{n} \cdot \vec{S}_1 \right)^2 \left( \hat{n} \cdot \vec{v}_1 \right)^2 - 18 \left( \hat{n} \cdot \vec{S}_1 \right)^2 \hat{n} \cdot \vec{v}_1 \hat{n} \cdot \vec{v}_2 + 3 \vec{v}_1 \cdot \vec{v}_2 \left( \hat{n} \cdot \vec{S}_1 \right)^2 - 6 \hat{n} \cdot \vec{S}_1 \hat{n} \cdot \vec{v}_1 \vec{S}_1 \cdot \vec{v}_1 + 6 \hat{n} \cdot \vec{S}_1 \hat{n} \cdot \vec{v}_1 \vec{S}_1 \cdot \vec{v}_2 - \right. \right.$$

$$\left. \left. 3 \vec{S}_1 \cdot \vec{S}_1 \left( \hat{n} \cdot \vec{v}_1 \right)^2 + 4 \vec{S}_1 \cdot \vec{S}_1 \hat{n} \cdot \vec{v}_1 \hat{n} \cdot \vec{v}_2 - \vec{S}_1 \cdot \vec{S}_1 \vec{v}_1 \cdot \vec{v}_2 \right) + \frac{2 \vec{S}_1 \cdot \vec{S}_1 \hat{n} \cdot \vec{v}_1 - 6 \hat{n} \cdot \vec{S}_1 \hat{n} \cdot \vec{S}_1 \hat{n} \cdot \vec{v}_1}{r^4} \right\}$$

{DiagS1CES2[3, 6, 39],

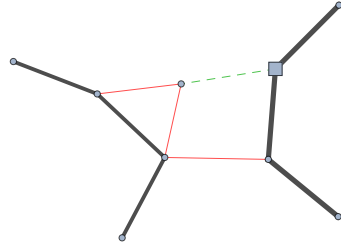

,

$$G^3 m_2^2 C_{ES^2_1} \left\{ \frac{1}{r^5} \left( 8 \left( \hat{n} \cdot \vec{S}_1 \right)^2 \left( \hat{n} \cdot \vec{v}_1 \right)^2 - 32 \left( \hat{n} \cdot \vec{S}_1 \right)^2 \hat{n} \cdot \vec{v}_1 \hat{n} \cdot \vec{v}_2 + 8 \vec{v}_1 \cdot \vec{v}_2 \left( \hat{n} \cdot \vec{S}_1 \right)^2 - \right. \right.$$

$$4 \hat{n} \cdot \vec{S}_1 \hat{n} \cdot \vec{v}_1 \vec{S}_1 \cdot \vec{v}_1 + 12 \hat{n} \cdot \vec{S}_1 \hat{n} \cdot \vec{v}_2 \vec{S}_1 \cdot \vec{v}_1 + 8 \hat{n} \cdot \vec{S}_1 \hat{n} \cdot \vec{v}_1 \vec{S}_1 \cdot \vec{v}_2 - 2 \vec{S}_1 \cdot \vec{v}_1 \vec{S}_1 \cdot \vec{v}_2 - 2 \vec{S}_1 \cdot \vec{S}_1 \vec{v}_1 \cdot \vec{v}_2 \left. \right) +$$

$$\frac{-4 \hat{n} \cdot \vec{S}_1 \hat{n} \cdot \vec{S}_1 \hat{n} \cdot \vec{v}_1 + 12 \hat{n} \cdot \vec{S}_1 \hat{n} \cdot \vec{S}_1 \hat{n} \cdot \vec{v}_2 - 3 \hat{n} \cdot \vec{S}_1 \vec{S}_1 \cdot \vec{v}_2 + 2 \vec{S}_1 \cdot \vec{S}_1 \hat{n} \cdot \vec{v}_2 - 3 \hat{n} \cdot \vec{S}_1 \vec{S}_1 \cdot \vec{v}_2}{r^4} \left. \right\}$$

{DiagS1CES2[3, 6, 40],

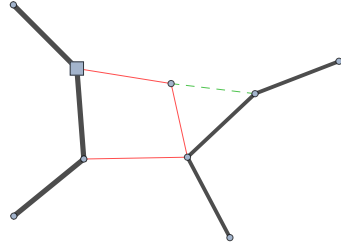

,

$$G^3 m_2^2 C_{ES^2_1} \left\{ \frac{1}{r^5} \left( 64 \left( \hat{n} \cdot \vec{S}_1 \right)^2 \left( \hat{n} \cdot \vec{v}_2 \right)^2 + 32 \left( \hat{n} \cdot \vec{S}_1 \right)^2 \hat{n} \cdot \vec{v}_1 \hat{n} \cdot \vec{v}_2 - 8 \vec{v}_1 \cdot \vec{v}_2 \left( \hat{n} \cdot \vec{S}_1 \right)^2 - 8 \vec{v}_2 \cdot \vec{v}_2 \left( \hat{n} \cdot \vec{S}_1 \right)^2 - \right. \right.$$

$$16 \hat{n} \cdot \vec{S}_1 \hat{n} \cdot \vec{v}_2 \vec{S}_1 \cdot \vec{v}_1 - 8 \hat{n} \cdot \vec{S}_1 \hat{n} \cdot \vec{v}_1 \vec{S}_1 \cdot \vec{v}_2 - 40 \hat{n} \cdot \vec{S}_1 \hat{n} \cdot \vec{v}_2 \vec{S}_1 \cdot \vec{v}_2 + 4 \left( \vec{S}_1 \cdot \vec{v}_2 \right)^2 + 4 \vec{S}_1 \cdot \vec{v}_1 \vec{S}_1 \cdot \vec{v}_2 \left. \right) +$$

$$\frac{-16 \hat{n} \cdot \vec{S}_1 \hat{n} \cdot \vec{S}_1 \hat{n} \cdot \vec{v}_2 + 4 \hat{n} \cdot \vec{S}_1 \vec{S}_1 \cdot \vec{v}_2 + 4 \hat{n} \cdot \vec{S}_1 \vec{S}_1 \cdot \vec{v}_2}{r^4} \left. \right\}$$

{DiagS1CES2[3, 6, 41],

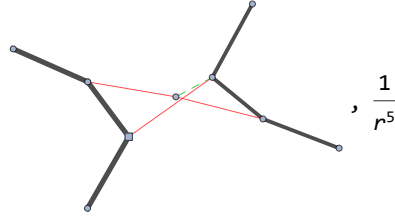

,  $\frac{1}{r^5}$

$$G^3 m_2^2 C_{ES^2 1} \left( 6 \left( \hat{n} \cdot \vec{S}_1 \right)^2 \left( \hat{n} \cdot \vec{v}_2 \right)^2 + 6 \left( \hat{n} \cdot \vec{S}_1 \right)^2 \hat{n} \cdot \vec{v}_1 \hat{n} \cdot \vec{v}_2 - 3 \vec{v}_1 \cdot \vec{v}_2 \left( \hat{n} \cdot \vec{S}_1 \right)^2 - \right. \\ \left. 3 \vec{v}_2 \cdot \vec{v}_2 \left( \hat{n} \cdot \vec{S}_1 \right)^2 - 2 \vec{S}_1 \cdot \vec{S}_1 \left( \hat{n} \cdot \vec{v}_2 \right)^2 - 2 \vec{S}_1 \cdot \vec{S}_1 \hat{n} \cdot \vec{v}_1 \hat{n} \cdot \vec{v}_2 + \vec{S}_1 \cdot \vec{S}_1 \vec{v}_1 \cdot \vec{v}_2 + \vec{S}_1 \cdot \vec{S}_1 \vec{v}_2 \cdot \vec{v}_2 \right) \Big\}$$

{DiagS1CES2[3, 6, 42],

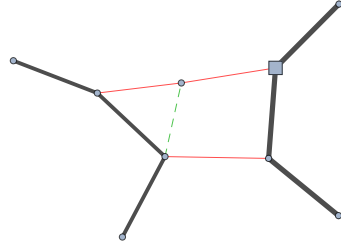

,

$$G^3 m_2^2 C_{ES^2 1} \left( \frac{1}{r^5} \left( 48 \left( \hat{n} \cdot \vec{S}_1 \right)^2 \left( \hat{n} \cdot \vec{v}_2 \right)^2 + 48 \left( \hat{n} \cdot \vec{S}_1 \right)^2 \hat{n} \cdot \vec{v}_1 \hat{n} \cdot \vec{v}_2 - 8 \vec{v}_1 \cdot \vec{v}_2 \left( \hat{n} \cdot \vec{S}_1 \right)^2 - 8 \vec{v}_2 \cdot \vec{v}_2 \left( \hat{n} \cdot \vec{S}_1 \right)^2 - \right. \right. \\ \left. \left. 16 \hat{n} \cdot \vec{S}_1 \hat{n} \cdot \vec{v}_2 \vec{S}_1 \cdot \vec{v}_1 - 16 \hat{n} \cdot \vec{S}_1 \hat{n} \cdot \vec{v}_1 \vec{S}_1 \cdot \vec{v}_2 - 32 \hat{n} \cdot \vec{S}_1 \hat{n} \cdot \vec{v}_2 \vec{S}_1 \cdot \vec{v}_2 + 4 \left( \vec{S}_1 \cdot \vec{v}_2 \right)^2 + 4 \vec{S}_1 \cdot \vec{v}_1 \vec{S}_1 \cdot \vec{v}_2 \right) + \right. \\ \left. \frac{-16 \hat{n} \cdot \vec{S}_1 \hat{n} \cdot \vec{S}_1 \hat{n} \cdot \vec{v}_2 + 4 \hat{n} \cdot \vec{S}_1 \vec{S}_1 \cdot \vec{v}_2 + 4 \hat{n} \cdot \vec{S}_1 \vec{S}_1 \cdot \vec{v}_2}{r^4} \right) \Big\}$$

{DiagS1CES2[3, 6, 43],

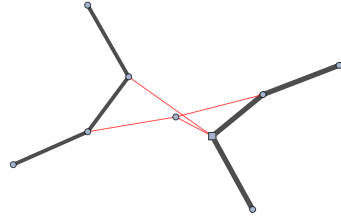

,

$$G^3 m_2^2 C_{ES^2 1} \left( \frac{1}{r^5} \left( \frac{315}{4} \left( \hat{n} \cdot \vec{S}_1 \right)^2 \left( \hat{n} \cdot \vec{v}_1 \right)^2 + 144 \left( \hat{n} \cdot \vec{S}_1 \right)^2 \left( \hat{n} \cdot \vec{v}_2 \right)^2 - 393 \left( \hat{n} \cdot \vec{S}_1 \right)^2 \hat{n} \cdot \vec{v}_1 \hat{n} \cdot \vec{v}_2 - \frac{45}{4} \vec{v}_1 \cdot \vec{v}_1 \left( \hat{n} \cdot \vec{S}_1 \right)^2 + \right. \right. \\ \left. \left. 48 \vec{v}_1 \cdot \vec{v}_2 \left( \hat{n} \cdot \vec{S}_1 \right)^2 - 45 \hat{n} \cdot \vec{S}_1 \hat{n} \cdot \vec{v}_1 \vec{S}_1 \cdot \vec{v}_1 + 108 \hat{n} \cdot \vec{S}_1 \hat{n} \cdot \vec{v}_2 \vec{S}_1 \cdot \vec{v}_1 + 96 \hat{n} \cdot \vec{S}_1 \hat{n} \cdot \vec{v}_1 \vec{S}_1 \cdot \vec{v}_2 - \right. \right. \\ \left. \left. 75 \hat{n} \cdot \vec{S}_1 \hat{n} \cdot \vec{v}_2 \vec{S}_1 \cdot \vec{v}_2 - \frac{45}{4} \vec{S}_1 \cdot \vec{S}_1 \left( \hat{n} \cdot \vec{v}_1 \right)^2 - 23 \vec{S}_1 \cdot \vec{S}_1 \left( \hat{n} \cdot \vec{v}_2 \right)^2 + 63 \vec{S}_1 \cdot \vec{S}_1 \hat{n} \cdot \vec{v}_1 \hat{n} \cdot \vec{v}_2 + \right. \right. \\ \left. \left. \frac{9}{2} \left( \vec{S}_1 \cdot \vec{v}_1 \right)^2 + 6 \left( \vec{S}_1 \cdot \vec{v}_2 \right)^2 - 18 \vec{S}_1 \cdot \vec{v}_1 \vec{S}_1 \cdot \vec{v}_2 + \frac{9}{4} \vec{S}_1 \cdot \vec{S}_1 \vec{v}_1 \cdot \vec{v}_1 - 10 \vec{S}_1 \cdot \vec{S}_1 \vec{v}_1 \cdot \vec{v}_2 - 2 \vec{S}_1 \cdot \vec{S}_1 \vec{v}_2 \cdot \vec{v}_2 \right) + \right. \\ \left. \frac{1}{r^4} \left( -30 \hat{n} \cdot \vec{S}_1 \hat{n} \cdot \vec{S}_1 \hat{n} \cdot \vec{v}_1 + 6 \vec{S}_1 \cdot \vec{S}_1 \hat{n} \cdot \vec{v}_1 + 96 \hat{n} \cdot \vec{S}_1 \hat{n} \cdot \vec{S}_1 \hat{n} \cdot \vec{v}_2 + 6 \hat{n} \cdot \vec{S}_1 \vec{S}_1 \cdot \vec{v}_1 - \right. \right. \\ \left. \left. 15 \hat{n} \cdot \vec{S}_1 \vec{S}_1 \cdot \vec{v}_2 - 30 \vec{S}_1 \cdot \vec{S}_1 \hat{n} \cdot \vec{v}_2 + 6 \hat{n} \cdot \vec{S}_1 \vec{S}_1 \cdot \vec{v}_1 - 15 \hat{n} \cdot \vec{S}_1 \vec{S}_1 \cdot \vec{v}_2 + 4 \vec{S}_1^2 \hat{n} \cdot \vec{v}_2 \right) \right) \Big\}$$

{DiagS1CES2[3, 6, 44],

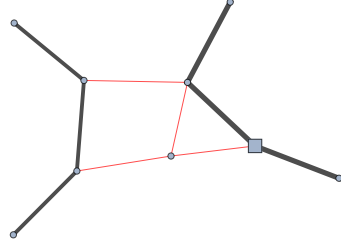

,  $G^3 m_2^2 C_{ES^2 1}$

$$\left\{ \frac{1}{r^5} \left( \frac{35}{4} (\hat{n} \cdot \vec{S}_1)^2 (\hat{n} \cdot \vec{v}_1)^2 + 6 (\hat{n} \cdot \vec{S}_1)^2 (\hat{n} \cdot \vec{v}_2)^2 - 47 (\hat{n} \cdot \vec{S}_1)^2 \hat{n} \cdot \vec{v}_1 \hat{n} \cdot \vec{v}_2 - \frac{5}{4} \vec{v}_1 \cdot \vec{v}_1 (\hat{n} \cdot \vec{S}_1)^2 + 6 \vec{v}_1 \cdot \vec{v}_2 (\hat{n} \cdot \vec{S}_1)^2 - \right. \right. \\ \left. 5 \hat{n} \cdot \vec{S}_1 \hat{n} \cdot \vec{v}_1 \vec{S}_1 \cdot \vec{v}_1 + 14 \hat{n} \cdot \vec{S}_1 \hat{n} \cdot \vec{v}_2 \vec{S}_1 \cdot \vec{v}_1 + 15 \hat{n} \cdot \vec{S}_1 \hat{n} \cdot \vec{v}_1 \vec{S}_1 \cdot \vec{v}_2 - 3 \hat{n} \cdot \vec{S}_1 \hat{n} \cdot \vec{v}_2 \vec{S}_1 \cdot \vec{v}_2 - \frac{5}{4} \vec{S}_1 \cdot \vec{S}_1 (\hat{n} \cdot \vec{v}_1)^2 - \right. \\ \left. \vec{S}_1 \cdot \vec{S}_1 (\hat{n} \cdot \vec{v}_2)^2 + 6 \vec{S}_1 \cdot \vec{S}_1 \hat{n} \cdot \vec{v}_1 \hat{n} \cdot \vec{v}_2 + \frac{1}{2} (\vec{S}_1 \cdot \vec{v}_1)^2 - 3 \vec{S}_1 \cdot \vec{v}_1 \vec{S}_1 \cdot \vec{v}_2 + \frac{1}{4} \vec{S}_1 \cdot \vec{S}_1 \vec{v}_1 \cdot \vec{v}_1 - \vec{S}_1 \cdot \vec{S}_1 \vec{v}_1 \cdot \vec{v}_2 \right) + \\ \left. \frac{1}{r^4} \left( -5 \hat{n} \cdot \vec{S}_1 \hat{n} \cdot \vec{S}_1 \hat{n} \cdot \vec{v}_1 + \vec{S}_1 \cdot \vec{S}_1 \hat{n} \cdot \vec{v}_1 + 15 \hat{n} \cdot \vec{S}_1 \hat{n} \cdot \vec{S}_1 \hat{n} \cdot \vec{v}_2 + \hat{n} \cdot \vec{S}_1 \vec{S}_1 \cdot \vec{v}_1 - \right. \right. \\ \left. \left. 3 \hat{n} \cdot \vec{S}_1 \vec{S}_1 \cdot \vec{v}_2 - 3 \vec{S}_1 \cdot \vec{S}_1 \hat{n} \cdot \vec{v}_2 + \hat{n} \cdot \vec{S}_1 \vec{S}_1 \cdot \vec{v}_1 - 3 \hat{n} \cdot \vec{S}_1 \vec{S}_1 \cdot \vec{v}_2 \right) \right\}$$

{DiagS1CES2[3, 6, 45],

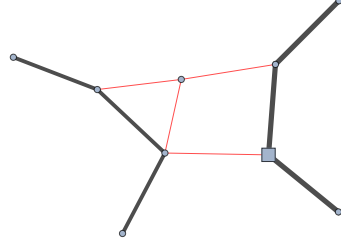

,

$$G^3 m_2^2 C_{ES^2 1} \left\{ \frac{1}{r^5} \left( 30 (\hat{n} \cdot \vec{S}_1)^2 (\hat{n} \cdot \vec{v}_1)^2 + \frac{33}{2} (\hat{n} \cdot \vec{S}_1)^2 (\hat{n} \cdot \vec{v}_2)^2 - 57 (\hat{n} \cdot \vec{S}_1)^2 \hat{n} \cdot \vec{v}_1 \hat{n} \cdot \vec{v}_2 + 6 \vec{v}_1 \cdot \vec{v}_2 (\hat{n} \cdot \vec{S}_1)^2 - \right. \right. \\ \left. \frac{3}{2} \vec{v}_2 \cdot \vec{v}_2 (\hat{n} \cdot \vec{S}_1)^2 - 12 \hat{n} \cdot \vec{S}_1 \hat{n} \cdot \vec{v}_1 \vec{S}_1 \cdot \vec{v}_1 + 6 \hat{n} \cdot \vec{S}_1 \hat{n} \cdot \vec{v}_2 \vec{S}_1 \cdot \vec{v}_1 + 12 \hat{n} \cdot \vec{S}_1 \hat{n} \cdot \vec{v}_1 \vec{S}_1 \cdot \vec{v}_2 - 6 \hat{n} \cdot \vec{S}_1 \hat{n} \cdot \vec{v}_2 \vec{S}_1 \cdot \vec{v}_2 - \right. \\ \left. 6 \vec{S}_1 \cdot \vec{S}_1 (\hat{n} \cdot \vec{v}_1)^2 - \frac{7}{2} \vec{S}_1 \cdot \vec{S}_1 (\hat{n} \cdot \vec{v}_2)^2 + 13 \vec{S}_1 \cdot \vec{S}_1 \hat{n} \cdot \vec{v}_1 \hat{n} \cdot \vec{v}_2 - 2 \vec{S}_1 \cdot \vec{S}_1 \vec{v}_1 \cdot \vec{v}_2 + \frac{1}{2} \vec{S}_1 \cdot \vec{S}_1 \vec{v}_2 \cdot \vec{v}_2 \right) + \\ \left. \frac{-12 \hat{n} \cdot \vec{S}_1 \hat{n} \cdot \vec{S}_1 \hat{n} \cdot \vec{v}_1 + 4 \vec{S}_1 \cdot \vec{S}_1 \hat{n} \cdot \vec{v}_1 + 6 \hat{n} \cdot \vec{S}_1 \hat{n} \cdot \vec{S}_1 \hat{n} \cdot \vec{v}_2 - 2 \vec{S}_1 \cdot \vec{S}_1 \hat{n} \cdot \vec{v}_2}{r^4} \right\}$$

{DiagS1CES2[3, 6, 46],

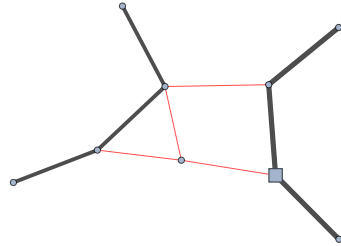

,

$$G^3 m_2^2 C_{ES^2 1} \left\{ \frac{1}{r^5} \left( 16 (\hat{n} \cdot \vec{S}_1)^2 (\hat{n} \cdot \vec{v}_1)^2 + 20 (\hat{n} \cdot \vec{S}_1)^2 (\hat{n} \cdot \vec{v}_2)^2 - 120 (\hat{n} \cdot \vec{S}_1)^2 \hat{n} \cdot \vec{v}_1 \hat{n} \cdot \vec{v}_2 + \right. \right. \\ \left. 16 \vec{v}_1 \cdot \vec{v}_2 (\hat{n} \cdot \vec{S}_1)^2 - 4 \vec{v}_2 \cdot \vec{v}_2 (\hat{n} \cdot \vec{S}_1)^2 - 8 \hat{n} \cdot \vec{S}_1 \hat{n} \cdot \vec{v}_1 \vec{S}_1 \cdot \vec{v}_1 + 40 \hat{n} \cdot \vec{S}_1 \hat{n} \cdot \vec{v}_2 \vec{S}_1 \cdot \vec{v}_1 + \right. \\ \left. 36 \hat{n} \cdot \vec{S}_1 \hat{n} \cdot \vec{v}_1 \vec{S}_1 \cdot \vec{v}_2 - 12 \hat{n} \cdot \vec{S}_1 \hat{n} \cdot \vec{v}_2 \vec{S}_1 \cdot \vec{v}_2 + (\vec{S}_1 \cdot \vec{v}_2)^2 - 8 \vec{S}_1 \cdot \vec{v}_1 \vec{S}_1 \cdot \vec{v}_2 + \vec{S}_1 \cdot \vec{S}_1 \vec{v}_2 \cdot \vec{v}_2 \right) +$$

$$\left. \frac{-8 \hat{n} \cdot \vec{S_1} \hat{n} \cdot \vec{S_1} \hat{n} \cdot \vec{v_1} + 40 \hat{n} \cdot \vec{S_1} \hat{n} \cdot \vec{S_1} \hat{n} \cdot \vec{v_2} - 8 \hat{n} \cdot \vec{S_1} \vec{S_1} \cdot \vec{v_2} - 8 \hat{n} \cdot \vec{S_1} \vec{S_1} \cdot \vec{v_2}}{\rho^4} \right\}$$

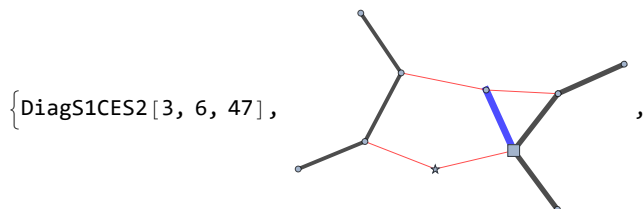

$$G^3 m_2^2 C_{ES^2 1} \left\{ \frac{1}{r^5} \left( 7 \left( \hat{n} \cdot \vec{S}_1 \right)^2 \left( \hat{n} \cdot \vec{v}_2 \right)^2 - \frac{21}{2} \left( \hat{n} \cdot \vec{S}_1 \right)^2 \hat{n} \cdot \vec{v}_1 \hat{n} \cdot \vec{v}_2 + \frac{3}{2} \vec{v}_1 \cdot \vec{v}_2 \left( \hat{n} \cdot \vec{S}_1 \right)^2 - 3 \vec{v}_2 \cdot \vec{v}_2 \left( \hat{n} \cdot \vec{S}_1 \right)^2 + \right. \right. \\ 3 \hat{n} \cdot \vec{S}_1 \hat{n} \cdot \vec{v}_2 \vec{S}_1 \cdot \vec{v}_1 + \frac{5}{2} \hat{n} \cdot \vec{S}_1 \hat{n} \cdot \vec{v}_1 \vec{S}_1 \cdot \vec{v}_2 - \frac{1}{2} \hat{n} \cdot \vec{S}_1 \hat{n} \cdot \vec{v}_2 \vec{S}_1 \cdot \vec{v}_2 - \frac{3}{2} \vec{S}_1 \cdot \vec{S}_1 \left( \hat{n} \cdot \vec{v}_2 \right)^2 - \\ 5 \vec{S}_1 \cdot \vec{S}_1 \hat{n} \cdot \vec{v}_1 \hat{n} \cdot \vec{v}_2 - \frac{3}{2} \left( \vec{S}_1 \cdot \vec{v}_2 \right)^2 - \frac{1}{2} \vec{S}_1 \cdot \vec{v}_1 \vec{S}_1 \cdot \vec{v}_2 + \vec{S}_1 \cdot \vec{S}_1 \vec{v}_1 \cdot \vec{v}_2 + \frac{7}{2} \vec{S}_1 \cdot \vec{S}_1 \vec{v}_2 \cdot \vec{v}_2 \Big) + \\ \left. \frac{3 \hat{n} \cdot \vec{S}_1 \hat{n} \cdot \vec{S}_1 \hat{n} \cdot \vec{v}_2 + 2 \vec{S}_1 \cdot \vec{S}_1 \hat{n} \cdot \vec{v}_2 - \frac{1}{2} \hat{n} \cdot \vec{S}_1 \vec{S}_1 \cdot \vec{v}_2 - \frac{1}{2} \hat{n} \cdot \vec{S}_1 \vec{S}_1 \cdot \vec{v}_2}{r^4} \right\}$$

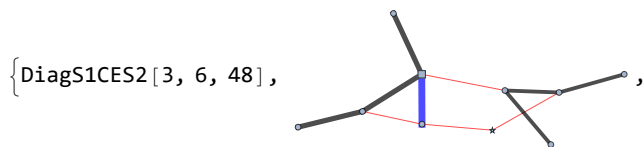

$$G^3 m_2^2 C_{\text{ES}^2} \left\{ \frac{1}{r^5} \left( \frac{49}{6} (\hat{n} \cdot \vec{S}_1)^2 (\hat{n} \cdot \vec{v}_2)^2 - \frac{49}{6} (\hat{n} \cdot \vec{S}_1)^2 \hat{n} \cdot \vec{v}_1 \hat{n} \cdot \vec{v}_2 + \frac{7}{6} \vec{v}_1 \cdot \vec{v}_2 (\hat{n} \cdot \vec{S}_1)^2 - \frac{13}{6} \vec{v}_2 \cdot \vec{v}_2 (\hat{n} \cdot \vec{S}_1)^2 + \right. \right. \\ \left. \frac{7}{3} \hat{n} \cdot \vec{S}_1 \hat{n} \cdot \vec{v}_2 \vec{S}_1 \cdot \vec{v}_1 - \frac{25}{6} \hat{n} \cdot \vec{S}_1 \hat{n} \cdot \vec{v}_1 \vec{S}_1 \cdot \vec{v}_2 + \frac{11}{6} \hat{n} \cdot \vec{S}_1 \hat{n} \cdot \vec{v}_2 \vec{S}_1 \cdot \vec{v}_2 - \frac{20}{3} \vec{S}_1 \cdot \vec{S}_1 (\hat{n} \cdot \vec{v}_2)^2 + \right. \\ \left. \frac{20}{3} \vec{S}_1 \cdot \vec{S}_1 \hat{n} \cdot \vec{v}_1 \hat{n} \cdot \vec{v}_2 - \frac{11}{6} (\vec{S}_1 \cdot \vec{v}_2)^2 + \frac{5}{6} \vec{S}_1 \cdot \vec{v}_1 \vec{S}_1 \cdot \vec{v}_2 - \frac{4}{3} \vec{S}_1 \cdot \vec{S}_1 \vec{v}_1 \cdot \vec{v}_2 + \frac{10}{3} \vec{S}_1 \cdot \vec{S}_1 \vec{v}_2 \cdot \vec{v}_2 \right) + \\ \left. \frac{\frac{7}{3} \hat{n} \cdot \vec{S}_1 \hat{n} \cdot \vec{S}_1 \hat{n} \cdot \vec{v}_2 - \frac{8}{3} \vec{S}_1 \cdot \vec{S}_1 \hat{n} \cdot \vec{v}_2 + \frac{5}{6} \hat{n} \cdot \vec{S}_1 \vec{S}_1 \cdot \vec{v}_2 + \frac{5}{6} \hat{n} \cdot \vec{S}_1 \vec{S}_1 \cdot \vec{v}_2}{r^4} \right\}$$

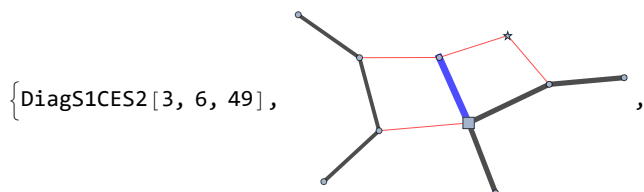

$$G^3 m_2^2 C_{\text{ES}^2_1} \left( \frac{1}{r^5} \left( \frac{215}{12} (\hat{n} \cdot \overline{S_1})^2 (\hat{n} \cdot \overline{v_1})^2 - \frac{259}{12} (\hat{n} \cdot \overline{S_1})^2 \hat{n} \cdot \overline{v_1} \hat{n} \cdot \overline{v_2} - \frac{47}{12} \overline{v_1} \cdot \overline{v_1} (\hat{n} \cdot \overline{S_1})^2 + \frac{37}{12} \overline{v_1} \cdot \overline{v_2} (\hat{n} \cdot \overline{S_1})^2 + \right. \right. \\ \left. \left. \frac{1}{3} \hat{n} \cdot \overline{S_1} \hat{n} \cdot \overline{v_1} \overline{S_1} \cdot \overline{v_1} - \frac{10}{3} \hat{n} \cdot \overline{S_1} \hat{n} \cdot \overline{v_2} \overline{S_1} \cdot \overline{v_1} + \frac{37}{6} \hat{n} \cdot \overline{S_1} \hat{n} \cdot \overline{v_1} \overline{S_1} \cdot \overline{v_2} - \frac{137}{12} \overline{S_1} \cdot \overline{S_1} (\hat{n} \cdot \overline{v_1})^2 + \right. \right.$$

$$\left. \frac{\frac{115}{12} \vec{S}_1 \cdot \vec{S}_1 \hat{n} \cdot \vec{v}_1 \hat{n} \cdot \vec{v}_2 - \frac{11}{6} (\vec{S}_1 \cdot \vec{v}_1)^2 + \frac{2}{3} \vec{S}_1 \cdot \vec{v}_1 \vec{S}_1 \cdot \vec{v}_2 + \frac{55}{12} \vec{S}_1 \cdot \vec{S}_1 \vec{v}_1 \cdot \vec{v}_1 - \frac{23}{12} \vec{S}_1 \cdot \vec{S}_1 \vec{v}_1 \cdot \vec{v}_2}{r^4} - \frac{37}{6} \hat{n} \cdot \vec{S}_1 \hat{n} \cdot \vec{S}_1 \hat{n} \cdot \vec{v}_1 + \frac{23}{6} \vec{S}_1 \cdot \vec{S}_1 \hat{n} \cdot \vec{v}_1 - \frac{2}{3} \hat{n} \cdot \vec{S}_1 \vec{S}_1 \cdot \vec{v}_1 - \frac{2}{3} \hat{n} \cdot \vec{S}_1 \vec{S}_1 \cdot \vec{v}_1} \right\}$$

{DiagS1CES2[3, 6, 50],

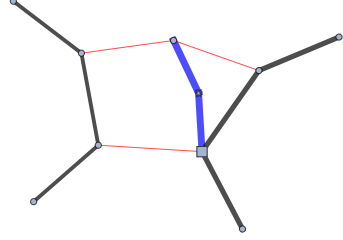

$$G^3 m_2^2 C_{ES^2 1} \left( \frac{1}{r^5} \left( -\frac{55}{12} (\hat{n} \cdot \vec{S}_1)^2 (\hat{n} \cdot \vec{v}_1)^2 - \frac{23}{3} (\hat{n} \cdot \vec{S}_1)^2 (\hat{n} \cdot \vec{v}_2)^2 + \frac{191}{12} (\hat{n} \cdot \vec{S}_1)^2 \hat{n} \cdot \vec{v}_1 \hat{n} \cdot \vec{v}_2 - \frac{5}{12} \vec{v}_1 \cdot \vec{v}_1 (\hat{n} \cdot \vec{S}_1)^2 - \frac{29}{12} \vec{v}_1 \cdot \vec{v}_2 (\hat{n} \cdot \vec{S}_1)^2 + \frac{5}{3} \vec{v}_2 \cdot \vec{v}_2 (\hat{n} \cdot \vec{S}_1)^2 + \frac{4}{3} \hat{n} \cdot \vec{S}_1 \hat{n} \cdot \vec{v}_1 \vec{S}_1 \cdot \vec{v}_1 - \frac{4}{3} \hat{n} \cdot \vec{S}_1 \hat{n} \cdot \vec{v}_2 \vec{S}_1 \cdot \vec{v}_1 - \frac{5}{6} \hat{n} \cdot \vec{S}_1 \hat{n} \cdot \vec{v}_1 \vec{S}_1 \cdot \vec{v}_2 - \frac{7}{3} \hat{n} \cdot \vec{S}_1 \hat{n} \cdot \vec{v}_2 \vec{S}_1 \cdot \vec{v}_2 + \frac{13}{12} \vec{S}_1 \cdot \vec{S}_1 (\hat{n} \cdot \vec{v}_1)^2 + \frac{20}{3} \vec{S}_1 \cdot \vec{S}_1 (\hat{n} \cdot \vec{v}_2)^2 - \frac{95}{12} \vec{S}_1 \cdot \vec{S}_1 \hat{n} \cdot \vec{v}_1 \hat{n} \cdot \vec{v}_2 + \frac{1}{6} (\vec{S}_1 \cdot \vec{v}_1)^2 + \frac{7}{3} (\vec{S}_1 \cdot \vec{v}_2)^2 - \frac{4}{3} \vec{S}_1 \cdot \vec{v}_1 \vec{S}_1 \cdot \vec{v}_2 + \frac{1}{12} \vec{S}_1 \cdot \vec{S}_1 \vec{v}_1 \cdot \vec{v}_1 + \frac{55}{12} \vec{S}_1 \cdot \vec{S}_1 \vec{v}_1 \cdot \vec{v}_2 - \frac{10}{3} \vec{S}_1 \cdot \vec{S}_1 \vec{v}_2 \cdot \vec{v}_2 \right) + \frac{1}{r^4} \left( -\frac{1}{2} \hat{n} \cdot \vec{S}_1 \hat{n} \cdot \vec{S}_1 \hat{n} \cdot \vec{v}_1 - \frac{1}{2} \vec{S}_1 \cdot \vec{S}_1 \hat{n} \cdot \vec{v}_1 - \frac{10}{3} \hat{n} \cdot \vec{S}_1 \hat{n} \cdot \vec{S}_1 \hat{n} \cdot \vec{v}_2 + \hat{n} \cdot \vec{S}_1 \vec{S}_1 \cdot \vec{v}_1 - \frac{1}{3} \hat{n} \cdot \vec{S}_1 \vec{S}_1 \cdot \vec{v}_2 + \frac{8}{3} \vec{S}_1 \cdot \vec{S}_1 \hat{n} \cdot \vec{v}_2 + \hat{n} \cdot \vec{S}_1 \vec{S}_1 \cdot \vec{v}_1 - \frac{1}{3} \hat{n} \cdot \vec{S}_1 \vec{S}_1 \cdot \vec{v}_2 \right) \right) \Bigg\}$$

{DiagS1CES2[3, 6, 51],

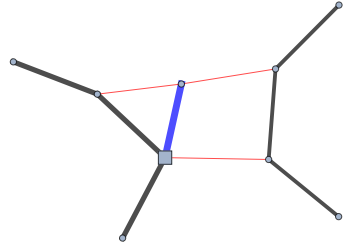

$$G^3 m_2^2 C_{ES^2 1} \left( \frac{-6 \hat{n} \cdot \vec{a}_1 (\hat{n} \cdot \vec{S}_1)^2 + 8 \hat{n} \cdot \vec{a}_2 (\hat{n} \cdot \vec{S}_1)^2 + \frac{5}{2} \vec{S}_1 \cdot \vec{a}_1 \hat{n} \cdot \vec{S}_1 - 4 \vec{S}_1 \cdot \vec{a}_2 \hat{n} \cdot \vec{S}_1 + \frac{1}{2} \vec{S}_1 \cdot \vec{S}_1 \hat{n} \cdot \vec{a}_1}{r^4} + \frac{1}{r^5} \left( 30 (\hat{n} \cdot \vec{S}_1)^2 (\hat{n} \cdot \vec{v}_1)^2 + 72 (\hat{n} \cdot \vec{S}_1)^2 (\hat{n} \cdot \vec{v}_2)^2 - 62 (\hat{n} \cdot \vec{S}_1)^2 \hat{n} \cdot \vec{v}_1 \hat{n} \cdot \vec{v}_2 - 18 \vec{v}_1 \cdot \vec{v}_1 (\hat{n} \cdot \vec{S}_1)^2 - 3 \vec{v}_1 \cdot \vec{v}_2 (\hat{n} \cdot \vec{S}_1)^2 - 17 \vec{v}_2 \cdot \vec{v}_2 (\hat{n} \cdot \vec{S}_1)^2 + \frac{17}{2} \hat{n} \cdot \vec{S}_1 \hat{n} \cdot \vec{v}_1 \vec{S}_1 \cdot \vec{v}_1 + \frac{7}{2} \hat{n} \cdot \vec{S}_1 \hat{n} \cdot \vec{v}_2 \vec{S}_1 \cdot \vec{v}_1 + 27 \hat{n} \cdot \vec{S}_1 \hat{n} \cdot \vec{v}_1 \vec{S}_1 \cdot \vec{v}_2 - 44 \hat{n} \cdot \vec{S}_1 \hat{n} \cdot \vec{v}_2 \vec{S}_1 \cdot \vec{v}_2 + \frac{9}{2} \vec{S}_1 \cdot \vec{S}_1 (\hat{n} \cdot \vec{v}_1)^2 - \frac{41}{2} \vec{S}_1 \cdot \vec{S}_1 \hat{n} \cdot \vec{v}_1 \hat{n} \cdot \vec{v}_2 - 3 (\vec{S}_1 \cdot \vec{v}_1)^2 + 4 (\vec{S}_1 \cdot \vec{v}_2)^2 - \frac{3}{2} \vec{S}_1 \cdot \vec{v}_1 \vec{S}_1 \cdot \vec{v}_2 + 13 \vec{S}_1 \cdot \vec{S}_1 \vec{v}_1 \cdot \vec{v}_1 + \frac{25}{2} \vec{S}_1 \cdot \vec{S}_1 \vec{v}_1 \cdot \vec{v}_2 + 15 \vec{S}_1 \cdot \vec{S}_1 \vec{v}_2 \cdot \vec{v}_2 \right) \right) \Bigg\}$$



$$\left\{ \text{DiagS1CES2}[3, 7, 1], \right. , \theta \left. \right\}$$
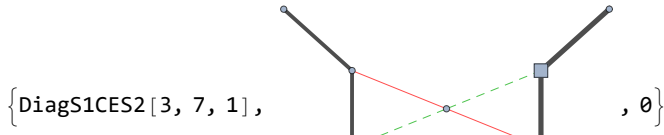

$$\left\{ \text{DiagS1CES2}[3, 7, 2], \right. , \theta \left. \right\}$$
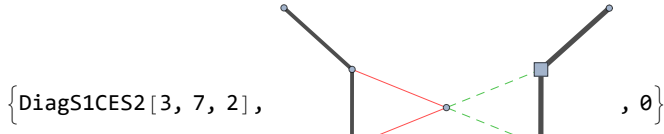

$$\left\{ \text{DiagS1CES2}[3, 7, 3], \right. , \theta \left. \right\}$$
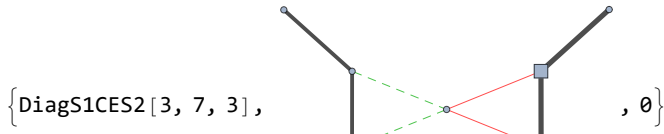

$$\left\{ \text{DiagS1CES2}[3, 7, 4], \right. , \theta \left. \right\}$$
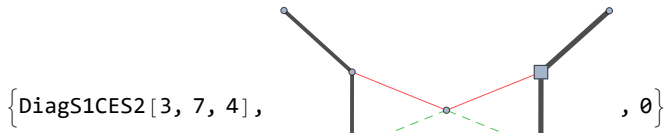

$$\left\{ \text{DiagS1CES2}[3, 7, 5], \right. , \left. \right\}$$
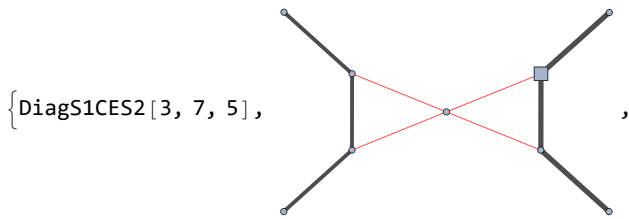

$$\begin{aligned} & \pi^2 G^3 m_2^2 C_{\text{ES}^2 1} \left( \frac{1}{r^5} \left( -\frac{525}{128} (\hat{n} \cdot \vec{S}_1)^2 (\hat{n} \cdot \vec{v}_1)^2 - \frac{315}{64} (\hat{n} \cdot \vec{S}_1)^2 (\hat{n} \cdot \vec{v}_2)^2 + \frac{315}{8} (\hat{n} \cdot \vec{S}_1)^2 \hat{n} \cdot \vec{v}_1 \hat{n} \cdot \vec{v}_2 + \right. \right. \\ & \quad \frac{75}{128} \vec{v}_1 \cdot \vec{v}_1 (\hat{n} \cdot \vec{S}_1)^2 - \frac{45}{8} \vec{v}_1 \cdot \vec{v}_2 (\hat{n} \cdot \vec{S}_1)^2 + \frac{45}{64} \vec{v}_2 \cdot \vec{v}_2 (\hat{n} \cdot \vec{S}_1)^2 + \frac{75}{32} \hat{n} \cdot \vec{S}_1 \hat{n} \cdot \vec{v}_1 \vec{S}_1 \cdot \vec{v}_1 - \\ & \quad \frac{45}{4} \hat{n} \cdot \vec{S}_1 \hat{n} \cdot \vec{v}_2 \vec{S}_1 \cdot \vec{v}_1 - \frac{45}{4} \hat{n} \cdot \vec{S}_1 \hat{n} \cdot \vec{v}_1 \vec{S}_1 \cdot \vec{v}_2 + \frac{45}{16} \hat{n} \cdot \vec{S}_1 \hat{n} \cdot \vec{v}_2 \vec{S}_1 \cdot \vec{v}_2 + \frac{75}{128} \vec{S}_1 \cdot \vec{S}_1 (\hat{n} \cdot \vec{v}_1)^2 + \\ & \quad \frac{45}{64} \vec{S}_1 \cdot \vec{S}_1 (\hat{n} \cdot \vec{v}_2)^2 - \frac{45}{8} \vec{S}_1 \cdot \vec{S}_1 \hat{n} \cdot \vec{v}_1 \hat{n} \cdot \vec{v}_2 - \frac{15}{64} (\vec{S}_1 \cdot \vec{v}_1)^2 - \frac{9}{32} (\vec{S}_1 \cdot \vec{v}_2)^2 + \frac{9}{4} \vec{S}_1 \cdot \vec{v}_1 \vec{S}_1 \cdot \vec{v}_2 - \\ & \quad \frac{15}{128} \vec{S}_1 \cdot \vec{S}_1 \vec{v}_1 \cdot \vec{v}_1 + \frac{9}{8} \vec{S}_1 \cdot \vec{S}_1 \vec{v}_1 \cdot \vec{v}_2 - \frac{9}{64} \vec{S}_1 \cdot \vec{S}_1 \vec{v}_2 \cdot \vec{v}_2 \left. \right) + \frac{1}{r^4} \left( \frac{15}{8} \hat{n} \cdot \vec{S}_1 \hat{n} \cdot \vec{S}_1 \hat{n} \cdot \vec{v}_1 - \frac{3}{8} \vec{S}_1 \cdot \vec{S}_1 \hat{n} \cdot \vec{v}_1 - \right. \\ & \quad \left. \frac{45}{4} \hat{n} \cdot \vec{S}_1 \hat{n} \cdot \vec{S}_1 \hat{n} \cdot \vec{v}_2 - \frac{3}{8} \hat{n} \cdot \vec{S}_1 \vec{S}_1 \cdot \vec{v}_1 + \frac{9}{4} \hat{n} \cdot \vec{S}_1 \vec{S}_1 \cdot \vec{v}_2 + \frac{9}{4} \vec{S}_1 \cdot \vec{S}_1 \hat{n} \cdot \vec{v}_2 - \frac{3}{8} \hat{n} \cdot \vec{S}_1 \vec{S}_1 \cdot \vec{v}_1 + \frac{9}{4} \hat{n} \cdot \vec{S}_1 \vec{S}_1 \cdot \vec{v}_2 \right) \left. \right) \Bigg\} \end{aligned}$$

$$\left\{ \text{DiagS1CES2}[3, 8, 1], \right. , \theta \left. \right\}$$
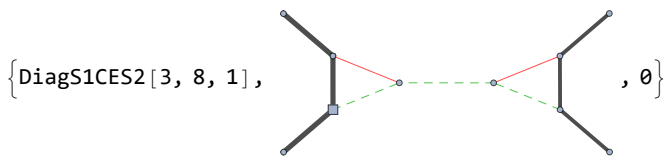

$$\left\{ \text{DiagS1CES2}[3, 8, 2], \right. , \left. \theta \right\}$$
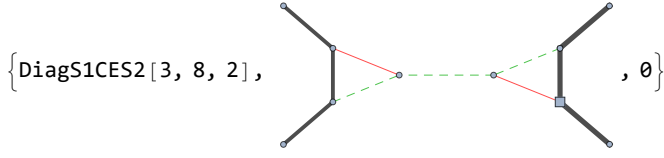

$$\left\{ \text{DiagS1CES2}[3, 8, 3], \right. ,$$
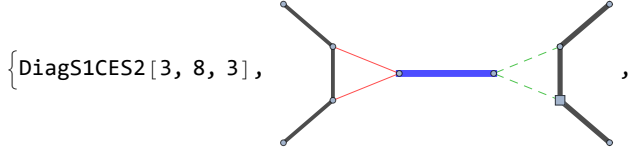

$$\pi^2 G^3 m_2^2 C_{\text{ES}^1} \left\{ \frac{1}{r^5} \left( -\frac{315}{64} (\hat{n} \cdot \vec{S}_1)^2 (\hat{n} \cdot \vec{v}_1)^2 + \frac{45}{64} \vec{v}_1 \cdot \vec{v}_1 (\hat{n} \cdot \vec{S}_1)^2 + \frac{45}{16} \hat{n} \cdot \vec{S}_1 \hat{n} \cdot \vec{v}_1 \vec{S}_1 \cdot \vec{v}_1 + \frac{45}{64} \vec{S}_1 \cdot \vec{S}_1 (\hat{n} \cdot \vec{v}_1)^2 - \right. \right.$$

$$\left. \frac{9}{32} (\vec{S}_1 \cdot \vec{v}_1)^2 - \frac{9}{64} \vec{S}_1 \cdot \vec{S}_1 \vec{v}_1 \cdot \vec{v}_1 \right) + \frac{\frac{15}{8} \hat{n} \cdot \vec{S}_1 \hat{n} \cdot \vec{S}_1 \hat{n} \cdot \vec{v}_1 - \frac{3}{8} \vec{S}_1 \cdot \vec{S}_1 \hat{n} \cdot \vec{v}_1 - \frac{3}{8} \hat{n} \cdot \vec{S}_1 \vec{S}_1 \cdot \vec{v}_1 - \frac{3}{8} \hat{n} \cdot \vec{S}_1 \vec{S}_1 \cdot \vec{v}_1}{r^4} \left. \right\}$$

$$\left\{ \text{DiagS1CES2}[3, 8, 4], \right. ,$$
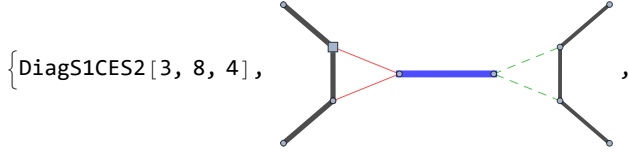

$$\frac{1}{r^5} \pi^2 G^3 m_2^2 C_{\text{ES}^1} \left( -\frac{525}{128} (\hat{n} \cdot \vec{S}_1)^2 (\hat{n} \cdot \vec{v}_2)^2 + \frac{75}{128} \vec{v}_2 \cdot \vec{v}_2 (\hat{n} \cdot \vec{S}_1)^2 + \right.$$

$$\left. \frac{75}{32} \hat{n} \cdot \vec{S}_1 \hat{n} \cdot \vec{v}_2 \vec{S}_1 \cdot \vec{v}_2 + \frac{75}{128} \vec{S}_1 \cdot \vec{S}_1 (\hat{n} \cdot \vec{v}_2)^2 - \frac{15}{64} (\vec{S}_1 \cdot \vec{v}_2)^2 - \frac{15}{128} \vec{S}_1 \cdot \vec{S}_1 \vec{v}_2 \cdot \vec{v}_2 \right\}$$

$$\left\{ \text{DiagS1CES2}[3, 8, 5], \right. ,$$
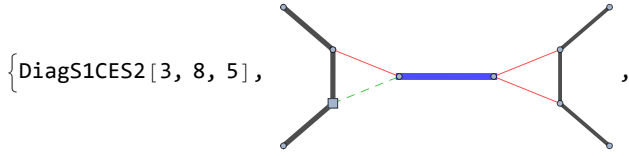

$$\pi^2 G^3 m_2^2 C_{\text{ES}^1} \left\{ \frac{1}{r^4} \left( \frac{15}{32} \hat{n} \cdot \vec{a}_1 (\hat{n} \cdot \vec{S}_1)^2 - \frac{3}{16} \vec{S}_1 \cdot \vec{a}_1 \hat{n} \cdot \vec{S}_1 - \frac{3}{32} \vec{S}_1 \cdot \vec{S}_1 \hat{n} \cdot \vec{a}_1 + \right. \right.$$

$$\left. \frac{15}{8} \hat{n} \cdot \vec{S}_1 \hat{n} \cdot \vec{S}_1 \hat{n} \cdot \vec{v}_1 - \frac{3}{8} \hat{n} \cdot \vec{S}_1 \vec{S}_1 \cdot \vec{v}_1 - \frac{3}{8} \vec{S}_1 \cdot \vec{S}_1 \hat{n} \cdot \vec{v}_1 - \frac{3}{8} \hat{n} \cdot \vec{S}_1 \vec{S}_1 \cdot \vec{v}_1 \right) + \frac{1}{r^5}$$

$$\left( -\frac{105}{32} (\hat{n} \cdot \vec{S}_1)^2 (\hat{n} \cdot \vec{v}_1)^2 + \frac{15}{32} \vec{v}_1 \cdot \vec{v}_1 (\hat{n} \cdot \vec{S}_1)^2 + \frac{15}{8} \hat{n} \cdot \vec{S}_1 \hat{n} \cdot \vec{v}_1 \vec{S}_1 \cdot \vec{v}_1 + \frac{15}{32} \vec{S}_1 \cdot \vec{S}_1 (\hat{n} \cdot \vec{v}_1)^2 - \right.$$

$$\left. \frac{3}{16} (\vec{S}_1 \cdot \vec{v}_1)^2 - \frac{3}{32} \vec{S}_1 \cdot \vec{S}_1 \vec{v}_1 \cdot \vec{v}_1 \right) + \frac{-\frac{3}{16} (\hat{n} \cdot \vec{S}_1)^2 - \frac{3}{16} \hat{n} \cdot \vec{S}_1 \hat{n} \cdot \vec{S}_1 + \frac{1}{16} \vec{S}_1 \cdot \vec{S}_1 + \frac{1}{16} \vec{S}_1 \cdot \vec{S}_1}{r^3} \left. \right\}$$

$$\left\{ \text{DiagS1CES2}[3, 8, 6], \right. ,$$
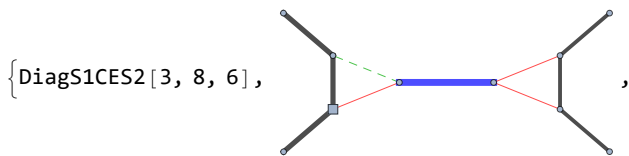

$$\pi^2 G^3 m_2^2 C_{ES^2 1} \left( \frac{1}{r^4} \left( -\frac{15}{32} \hat{n} \cdot \vec{a}_1 \left( \hat{n} \cdot \vec{S}_1 \right)^2 + \frac{3}{16} \vec{S}_1 \cdot \vec{a}_1 \hat{n} \cdot \vec{S}_1 + \frac{3}{32} \vec{S}_1 \cdot \vec{S}_1 \hat{n} \cdot \vec{a}_1 - \frac{15}{16} \hat{n} \cdot \vec{S}_1 \hat{n} \cdot \vec{S}_1 \hat{n} \cdot \vec{v}_1 + \right. \right. \\ \left. \left. \frac{3}{16} \hat{n} \cdot \vec{S}_1 \frac{1}{S_1} \cdot \vec{v}_1 + \frac{3}{16} \vec{S}_1 \cdot \frac{1}{S_1} \hat{n} \cdot \vec{v}_1 + \frac{3}{16} \hat{n} \cdot \frac{1}{S_1} \vec{S}_1 \cdot \vec{v}_1 \right) + \frac{1}{r^5} \left( \frac{105}{32} \left( \hat{n} \cdot \vec{S}_1 \right)^2 \left( \hat{n} \cdot \vec{v}_1 \right)^2 - \right. \right. \\ \left. \left. \frac{15}{32} \vec{v}_1 \cdot \vec{v}_1 \left( \hat{n} \cdot \vec{S}_1 \right)^2 - \frac{15}{8} \hat{n} \cdot \vec{S}_1 \hat{n} \cdot \vec{v}_1 \vec{S}_1 \cdot \vec{v}_1 - \frac{15}{32} \vec{S}_1 \cdot \vec{S}_1 \left( \hat{n} \cdot \vec{v}_1 \right)^2 + \frac{3}{16} \left( \vec{S}_1 \cdot \vec{v}_1 \right)^2 + \frac{3}{32} \vec{S}_1 \cdot \vec{S}_1 \vec{v}_1 \cdot \vec{v}_1 \right) \right) \Bigg\}$$

$$\left\{ \text{DiagS1CES2}[3, 8, 7], \right. \\ \left. \right\}, \emptyset \}$$
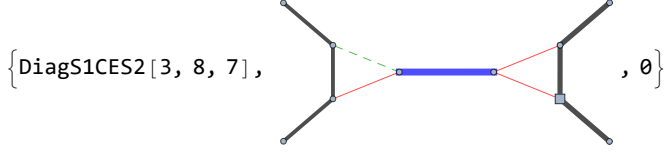

$$\left\{ \text{DiagS1CES2}[3, 8, 8], \right. \\ \left. \right\},$$
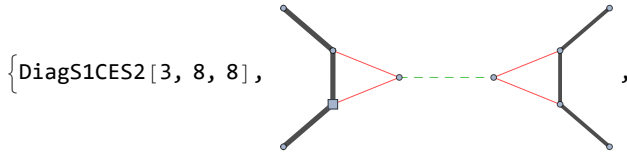

$$\pi^2 G^3 m_2^2 C_{ES^2 1} \left( \frac{1}{r^5} \left( -\frac{1785 \left( \hat{n} \cdot \vec{S}_1 \right)^2 \hat{n} \cdot \vec{v}_1 \hat{n} \cdot \vec{v}_2}{1024} + \frac{255 \vec{v}_1 \cdot \vec{v}_2 \left( \hat{n} \cdot \vec{S}_1 \right)^2}{1024} + \frac{255}{512} \hat{n} \cdot \vec{S}_1 \hat{n} \cdot \vec{v}_2 \vec{S}_1 \cdot \vec{v}_1 + \right. \right. \\ \left. \left. \frac{255}{512} \hat{n} \cdot \vec{S}_1 \hat{n} \cdot \vec{v}_1 \vec{S}_1 \cdot \vec{v}_2 + \frac{255 \vec{S}_1 \cdot \vec{S}_1 \hat{n} \cdot \vec{v}_1 \hat{n} \cdot \vec{v}_2}{1024} - \frac{51}{512} \vec{S}_1 \cdot \vec{v}_1 \vec{S}_1 \cdot \vec{v}_2 - \frac{51 \vec{S}_1 \cdot \vec{S}_1 \vec{v}_1 \cdot \vec{v}_2}{1024} \right) + \right. \\ \left. \frac{\frac{15}{32} \hat{n} \cdot \vec{S}_1 \frac{1}{S_1} \hat{n} \cdot \vec{S}_1 \hat{n} \cdot \vec{v}_2 - \frac{3}{32} \vec{S}_1 \cdot \frac{1}{S_1} \hat{n} \cdot \vec{v}_2 - \frac{3}{32} \hat{n} \cdot \vec{S}_1 \frac{1}{S_1} \vec{S}_1 \cdot \vec{v}_2 - \frac{3}{32} \hat{n} \cdot \vec{S}_1 \frac{1}{S_1} \vec{S}_1 \cdot \vec{v}_2}{r^4} \right) \Bigg\}$$

$$\left\{ \text{DiagS1CES2}[3, 8, 9], \right. \\ \left. \right\}, \frac{1}{r^5}$$
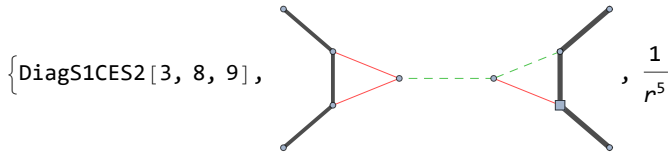

$$\pi^2 G^3 m_2^2 C_{ES^2 1} \left( \frac{105}{64} \left( \hat{n} \cdot \vec{S}_1 \right)^2 \hat{n} \cdot \vec{v}_1 \hat{n} \cdot \vec{v}_2 - \frac{15}{64} \vec{v}_1 \cdot \vec{v}_2 \left( \hat{n} \cdot \vec{S}_1 \right)^2 - \frac{15}{32} \hat{n} \cdot \vec{S}_1 \hat{n} \cdot \vec{v}_2 \vec{S}_1 \cdot \vec{v}_1 - \right. \\ \left. \frac{15}{32} \hat{n} \cdot \vec{S}_1 \hat{n} \cdot \vec{v}_1 \vec{S}_1 \cdot \vec{v}_2 - \frac{15}{64} \vec{S}_1 \cdot \vec{S}_1 \hat{n} \cdot \vec{v}_1 \hat{n} \cdot \vec{v}_2 + \frac{3}{32} \vec{S}_1 \cdot \vec{v}_1 \vec{S}_1 \cdot \vec{v}_2 + \frac{3}{64} \vec{S}_1 \cdot \vec{S}_1 \vec{v}_1 \cdot \vec{v}_2 \right) \Bigg\}$$

$$\left\{ \text{DiagS1CES2}[3, 8, 10], \right. \\ \left. \right\},$$
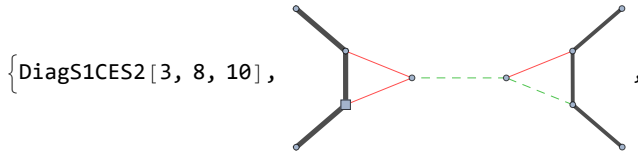

$$\pi^2 G^3 m_2^2 C_{ES^2 1} \left( \frac{1}{r^5} \left( \frac{525}{64} \left( \hat{n} \cdot \vec{S}_1 \right)^2 \hat{n} \cdot \vec{v}_1 \hat{n} \cdot \vec{v}_2 - \frac{75}{64} \vec{v}_1 \cdot \vec{v}_2 \left( \hat{n} \cdot \vec{S}_1 \right)^2 - \frac{75}{32} \hat{n} \cdot \vec{S}_1 \hat{n} \cdot \vec{v}_2 \vec{S}_1 \cdot \vec{v}_1 - \right. \right. \\ \left. \left. \frac{75}{32} \hat{n} \cdot \vec{S}_1 \hat{n} \cdot \vec{v}_1 \vec{S}_1 \cdot \vec{v}_2 - \frac{75}{64} \vec{S}_1 \cdot \vec{S}_1 \hat{n} \cdot \vec{v}_1 \hat{n} \cdot \vec{v}_2 + \frac{15}{32} \vec{S}_1 \cdot \vec{v}_1 \vec{S}_1 \cdot \vec{v}_2 + \frac{15}{64} \vec{S}_1 \cdot \vec{S}_1 \vec{v}_1 \cdot \vec{v}_2 \right) + \right. \\ \left. \frac{-\frac{15}{8} \hat{n} \cdot \vec{S}_1 \frac{1}{S_1} \hat{n} \cdot \vec{S}_1 \hat{n} \cdot \vec{v}_2 + \frac{3}{8} \vec{S}_1 \cdot \frac{1}{S_1} \hat{n} \cdot \vec{v}_2 + \frac{3}{8} \hat{n} \cdot \vec{S}_1 \frac{1}{S_1} \vec{S}_1 \cdot \vec{v}_2 + \frac{3}{8} \hat{n} \cdot \vec{S}_1 \frac{1}{S_1} \vec{S}_1 \cdot \vec{v}_2}{r^4} \right) \Bigg\}$$

$\{\text{DiagS1CES2}[3, 8, 11],$

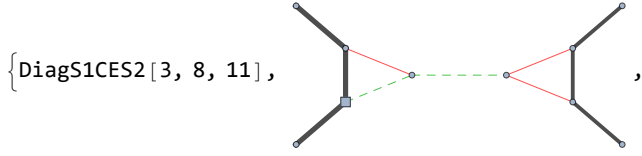

,

$$\pi^2 G^3 m_2^2 C_{\text{ES}^2} \left\{ \frac{1}{r^5} \left( \frac{525}{64} (\hat{n} \cdot \vec{S}_1)^2 \hat{n} \cdot \vec{v}_1 \hat{n} \cdot \vec{v}_2 - \frac{75}{64} \vec{v}_1 \cdot \vec{v}_2 (\hat{n} \cdot \vec{S}_1)^2 - \frac{75}{32} \hat{n} \cdot \vec{S}_1 \hat{n} \cdot \vec{v}_2 \vec{S}_1 \cdot \vec{v}_1 - \frac{75}{32} \hat{n} \cdot \vec{S}_1 \hat{n} \cdot \vec{v}_1 \vec{S}_1 \cdot \vec{v}_2 - \frac{75}{64} \vec{S}_1 \cdot \vec{S}_1 \hat{n} \cdot \vec{v}_1 \hat{n} \cdot \vec{v}_2 + \frac{15}{32} \vec{S}_1 \cdot \vec{v}_1 \vec{S}_1 \cdot \vec{v}_2 + \frac{15}{64} \vec{S}_1 \cdot \vec{S}_1 \vec{v}_1 \cdot \vec{v}_2 \right) + \frac{-\frac{45}{16} \hat{n} \cdot \vec{S}_1 \hat{n} \cdot \vec{S}_1 \hat{n} \cdot \vec{v}_2 + \frac{9}{16} \vec{S}_1 \cdot \vec{S}_1 \hat{n} \cdot \vec{v}_2 + \frac{9}{16} \hat{n} \cdot \vec{S}_1 \vec{S}_1 \cdot \vec{v}_2 + \frac{9}{16} \hat{n} \cdot \vec{S}_1 \vec{S}_1 \cdot \vec{v}_2}{r^4} \right\}$$

$\{\text{DiagS1CES2}[3, 8, 12],$

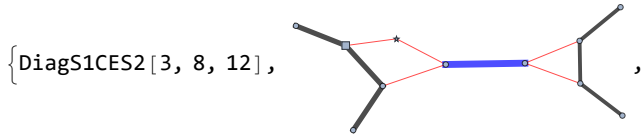

,

$$\pi^2 G^3 m_2^2 C_{\text{ES}^2} \left\{ \frac{1}{r^5} \left( -\frac{315 (\hat{n} \cdot \vec{S}_1)^2 (\hat{n} \cdot \vec{v}_1)^2}{4096} + \frac{735 (\hat{n} \cdot \vec{S}_1)^2 \hat{n} \cdot \vec{v}_1 \hat{n} \cdot \vec{v}_2}{1024} + \frac{45 \vec{v}_1 \cdot \vec{v}_1 (\hat{n} \cdot \vec{S}_1)^2}{4096} - \frac{105 \vec{v}_1 \cdot \vec{v}_2 (\hat{n} \cdot \vec{S}_1)^2}{1024} + \frac{45 \hat{n} \cdot \vec{S}_1 \hat{n} \cdot \vec{v}_1 \vec{S}_1 \cdot \vec{v}_1}{1024} - \frac{105}{512} \hat{n} \cdot \vec{S}_1 \hat{n} \cdot \vec{v}_2 \vec{S}_1 \cdot \vec{v}_1 - \frac{105}{512} \hat{n} \cdot \vec{S}_1 \hat{n} \cdot \vec{v}_1 \vec{S}_1 \cdot \vec{v}_2 + \frac{45 \vec{S}_1 \cdot \vec{S}_1 (\hat{n} \cdot \vec{v}_1)^2}{4096} - \frac{105 \vec{S}_1 \cdot \vec{S}_1 \hat{n} \cdot \vec{v}_1 \hat{n} \cdot \vec{v}_2}{1024} - \frac{9 (\vec{S}_1 \cdot \vec{v}_1)^2}{2048} + \frac{21}{512} \vec{S}_1 \cdot \vec{v}_1 \vec{S}_1 \cdot \vec{v}_2 - \frac{9 \vec{S}_1 \cdot \vec{S}_1 \vec{v}_1 \cdot \vec{v}_1}{4096} + \frac{21 \vec{S}_1 \cdot \vec{S}_1 \vec{v}_1 \cdot \vec{v}_2}{1024} \right) + \frac{1}{r^4} \left( \frac{15}{512} \hat{n} \cdot \vec{S}_1 \hat{n} \cdot \vec{S}_1 \hat{n} \cdot \vec{v}_1 - \frac{3}{512} \vec{S}_1 \cdot \vec{S}_1 \hat{n} \cdot \vec{v}_1 - \frac{15}{64} \hat{n} \cdot \vec{S}_1 \hat{n} \cdot \vec{S}_1 \hat{n} \cdot \vec{v}_2 - \frac{3}{512} \hat{n} \cdot \vec{S}_1 \vec{S}_1 \cdot \vec{v}_1 + \frac{3}{64} \hat{n} \cdot \vec{S}_1 \vec{S}_1 \cdot \vec{v}_2 + \frac{3}{64} \vec{S}_1 \cdot \vec{S}_1 \hat{n} \cdot \vec{v}_2 - \frac{3}{512} \hat{n} \cdot \vec{S}_1 \vec{S}_1 \cdot \vec{v}_1 + \frac{3}{64} \hat{n} \cdot \vec{S}_1 \vec{S}_1 \cdot \vec{v}_2 \right) \right\}$$

$\{\text{DiagS1CES2}[3, 8, 13],$

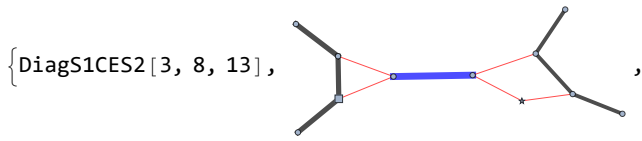

,

$$\pi^2 G^3 m_2^2 C_{\text{ES}^2} \left\{ \frac{1}{r^5} \left( -\frac{105 (\hat{n} \cdot \vec{S}_1)^2 (\hat{n} \cdot \vec{v}_2)^2}{2048} + \frac{315 (\hat{n} \cdot \vec{S}_1)^2 \hat{n} \cdot \vec{v}_1 \hat{n} \cdot \vec{v}_2}{512} - \frac{45}{512} \vec{v}_1 \cdot \vec{v}_2 (\hat{n} \cdot \vec{S}_1)^2 + \frac{15 \vec{v}_2 \cdot \vec{v}_2 (\hat{n} \cdot \vec{S}_1)^2}{2048} - \frac{45}{256} \hat{n} \cdot \vec{S}_1 \hat{n} \cdot \vec{v}_2 \vec{S}_1 \cdot \vec{v}_1 - \frac{45}{256} \hat{n} \cdot \vec{S}_1 \hat{n} \cdot \vec{v}_1 \vec{S}_1 \cdot \vec{v}_2 + \frac{15}{512} \hat{n} \cdot \vec{S}_1 \hat{n} \cdot \vec{v}_2 \vec{S}_1 \cdot \vec{v}_2 + \frac{15 \vec{S}_1 \cdot \vec{S}_1 (\hat{n} \cdot \vec{v}_2)^2}{2048} - \frac{45}{512} \vec{S}_1 \cdot \vec{S}_1 \hat{n} \cdot \vec{v}_1 \hat{n} \cdot \vec{v}_2 - \frac{3 (\vec{S}_1 \cdot \vec{v}_2)^2}{1024} + \frac{9}{256} \vec{S}_1 \cdot \vec{v}_1 \vec{S}_1 \cdot \vec{v}_2 + \frac{9}{512} \vec{S}_1 \cdot \vec{S}_1 \vec{v}_1 \cdot \vec{v}_2 - \frac{3 \vec{S}_1 \cdot \vec{S}_1 \vec{v}_2 \cdot \vec{v}_2}{2048} \right) + \frac{-\frac{45}{256} \hat{n} \cdot \vec{S}_1 \hat{n} \cdot \vec{S}_1 \hat{n} \cdot \vec{v}_2 + \frac{9}{256} \vec{S}_1 \cdot \vec{S}_1 \hat{n} \cdot \vec{v}_2 + \frac{9}{256} \hat{n} \cdot \vec{S}_1 \vec{S}_1 \cdot \vec{v}_2 + \frac{9}{256} \hat{n} \cdot \vec{S}_1 \vec{S}_1 \cdot \vec{v}_2}{r^4} \right\}$$

$\{\text{DiagS1CES2}[3, 8, 14],$

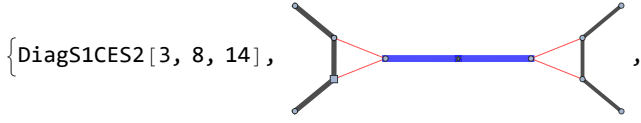

,

$$\pi^2 G^3 m_2^2 C_{\text{ES}^2} \left\{ \frac{1}{r^5} \left( -\frac{315}{512} (\hat{n} \cdot \vec{S}_1)^2 \hat{n} \cdot \vec{v}_1 \hat{n} \cdot \vec{v}_2 + \frac{45}{512} \vec{v}_1 \cdot \vec{v}_2 (\hat{n} \cdot \vec{S}_1)^2 + \frac{45}{256} \hat{n} \cdot \vec{S}_1 \hat{n} \cdot \vec{v}_2 \vec{S}_1 \cdot \vec{v}_1 + \right. \right.$$

$$\left. \frac{45}{256} \hat{n} \cdot \vec{S}_1 \hat{n} \cdot \vec{v}_1 \vec{S}_1 \cdot \vec{v}_2 + \frac{45}{512} \vec{S}_1 \cdot \vec{S}_1 \hat{n} \cdot \vec{v}_1 \hat{n} \cdot \vec{v}_2 - \frac{9}{256} \vec{S}_1 \cdot \vec{v}_1 \vec{S}_1 \cdot \vec{v}_2 - \frac{9}{512} \vec{S}_1 \cdot \vec{S}_1 \vec{v}_1 \cdot \vec{v}_2 \right) +$$

$$\left. \frac{\frac{45}{256} \hat{n} \cdot \vec{S}_1 \hat{n} \cdot \vec{S}_1 \hat{n} \cdot \vec{v}_2 - \frac{9}{256} \vec{S}_1 \cdot \vec{S}_1 \hat{n} \cdot \vec{v}_2 - \frac{9}{256} \hat{n} \cdot \vec{S}_1 \vec{S}_1 \cdot \vec{v}_2 - \frac{9}{256} \hat{n} \cdot \vec{S}_1 \vec{S}_1 \cdot \vec{v}_2}{r^4} \right\}$$

$\{\text{DiagS1CES2}[3, 8, 15],$

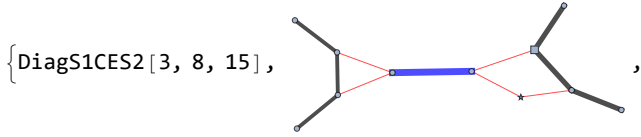

,

$$\pi^2 G^3 m_2^2 C_{\text{ES}^2} \left\{ \frac{1}{r^5} \left( \frac{525 (\hat{n} \cdot \vec{S}_1)^2 (\hat{n} \cdot \vec{v}_1)^2}{4096} - \frac{105 (\hat{n} \cdot \vec{S}_1)^2 \hat{n} \cdot \vec{v}_1 \hat{n} \cdot \vec{v}_2}{1024} - \frac{75 \vec{v}_1 \cdot \vec{v}_1 (\hat{n} \cdot \vec{S}_1)^2}{4096} + \frac{15 \vec{v}_1 \cdot \vec{v}_2 (\hat{n} \cdot \vec{S}_1)^2}{1024} - \right. \right.$$

$$\frac{75 \hat{n} \cdot \vec{S}_1 \hat{n} \cdot \vec{v}_1 \vec{S}_1 \cdot \vec{v}_1}{1024} + \frac{15}{512} \hat{n} \cdot \vec{S}_1 \hat{n} \cdot \vec{v}_2 \vec{S}_1 \cdot \vec{v}_1 + \frac{15}{512} \hat{n} \cdot \vec{S}_1 \hat{n} \cdot \vec{v}_1 \vec{S}_1 \cdot \vec{v}_2 - \frac{75 \vec{S}_1 \cdot \vec{S}_1 (\hat{n} \cdot \vec{v}_1)^2}{4096} +$$

$$\frac{15 \vec{S}_1 \cdot \vec{S}_1 \hat{n} \cdot \vec{v}_1 \hat{n} \cdot \vec{v}_2}{1024} + \frac{15 (\vec{S}_1 \cdot \vec{v}_1)^2}{2048} - \frac{3}{512} \vec{S}_1 \cdot \vec{v}_1 \vec{S}_1 \cdot \vec{v}_2 + \frac{15 \vec{S}_1 \cdot \vec{S}_1 \vec{v}_1 \cdot \vec{v}_1}{4096} - \frac{3 \vec{S}_1 \cdot \vec{S}_1 \vec{v}_1 \cdot \vec{v}_2}{1024} \left. \right) +$$

$$\left. \frac{-\frac{15}{512} \hat{n} \cdot \vec{S}_1 \hat{n} \cdot \vec{S}_1 \hat{n} \cdot \vec{v}_1 + \frac{3}{512} \vec{S}_1 \cdot \vec{S}_1 \hat{n} \cdot \vec{v}_1 + \frac{3}{512} \hat{n} \cdot \vec{S}_1 \vec{S}_1 \cdot \vec{v}_1 + \frac{3}{512} \hat{n} \cdot \vec{S}_1 \vec{S}_1 \cdot \vec{v}_1}{r^4} \right\}$$

$\{\text{DiagS1CES2}[3, 8, 16],$

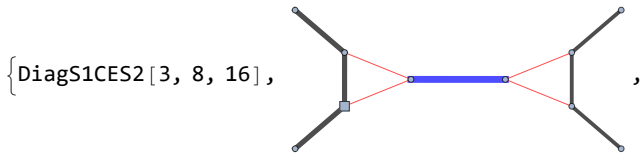

,

$$\pi^2 G^3 m_2^2 C_{\text{ES}^2} \left\{ \frac{1}{r^5} \left( \frac{525 (\hat{n} \cdot \vec{S}_1)^2 (\hat{n} \cdot \vec{v}_1)^2}{1024} + \frac{315}{512} (\hat{n} \cdot \vec{S}_1)^2 (\hat{n} \cdot \vec{v}_2)^2 - \frac{75 \vec{v}_1 \cdot \vec{v}_1 (\hat{n} \cdot \vec{S}_1)^2}{1024} - \right. \right.$$

$$\frac{45}{512} \vec{v}_2 \cdot \vec{v}_2 (\hat{n} \cdot \vec{S}_1)^2 - \frac{75}{256} \hat{n} \cdot \vec{S}_1 \hat{n} \cdot \vec{v}_1 \vec{S}_1 \cdot \vec{v}_1 - \frac{45}{128} \hat{n} \cdot \vec{S}_1 \hat{n} \cdot \vec{v}_2 \vec{S}_1 \cdot \vec{v}_2 - \frac{75 \vec{S}_1 \cdot \vec{S}_1 (\hat{n} \cdot \vec{v}_1)^2}{1024} -$$

$$\frac{45}{512} \vec{S}_1 \cdot \vec{S}_1 (\hat{n} \cdot \vec{v}_2)^2 + \frac{15}{512} (\vec{S}_1 \cdot \vec{v}_1)^2 + \frac{9}{256} (\vec{S}_1 \cdot \vec{v}_2)^2 + \frac{15 \vec{S}_1 \cdot \vec{S}_1 \vec{v}_1 \cdot \vec{v}_1}{1024} + \frac{9}{512} \vec{S}_1 \cdot \vec{S}_1 \vec{v}_2 \cdot \vec{v}_2 \left. \right) +$$

$$\left. \frac{-\frac{15}{64} \hat{n} \cdot \vec{S}_1 \hat{n} \cdot \vec{S}_1 \hat{n} \cdot \vec{v}_1 + \frac{3}{64} \vec{S}_1 \cdot \vec{S}_1 \hat{n} \cdot \vec{v}_1 + \frac{3}{64} \hat{n} \cdot \vec{S}_1 \vec{S}_1 \cdot \vec{v}_1 + \frac{3}{64} \hat{n} \cdot \vec{S}_1 \vec{S}_1 \cdot \vec{v}_1}{r^4} \right\}$$

{DiagS1CES2[3, 9, 1],

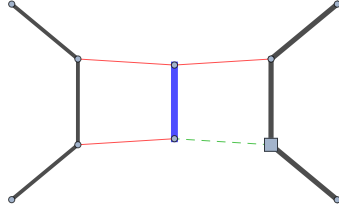

,

$$\begin{aligned}
 G^3 & \left( \frac{22 \left( \hat{n} \cdot \vec{S}_1 \right)^2 + 22 \hat{n} \cdot \vec{S}_1 \hat{n} \cdot \vec{S}_1 - 18 \vec{S}_1 \cdot \vec{S}_1 - 18 \vec{S}_1 \cdot \vec{S}_1}{r^3} + \frac{1}{r^4} \right. \\
 & \left( -29 \hat{n} \cdot \vec{a}_1 \left( \hat{n} \cdot \vec{S}_1 \right)^2 - 116 \hat{n} \cdot \vec{S}_1 \hat{n} \cdot \vec{v}_1 \hat{n} \cdot \vec{S}_1 + 84 \hat{n} \cdot \vec{S}_1 \hat{n} \cdot \vec{v}_2 \hat{n} \cdot \vec{S}_1 + 16 \vec{S}_1 \cdot \vec{v}_1 \hat{n} \cdot \vec{S}_1 - 18 \vec{S}_1 \cdot \vec{v}_2 \hat{n} \cdot \vec{S}_1 + \right. \\
 & \left. 2 \vec{S}_1 \cdot \vec{a}_1 \hat{n} \cdot \vec{S}_1 + 28 \hat{n} \cdot \vec{v}_1 \vec{S}_1 \cdot \vec{S}_1 - 32 \hat{n} \cdot \vec{v}_2 \vec{S}_1 \cdot \vec{S}_1 + \hat{n} \cdot \vec{a}_1 \vec{S}_1 \cdot \vec{S}_1 + 16 \hat{n} \cdot \vec{S}_1 \vec{S}_1 \cdot \vec{v}_1 - 18 \hat{n} \cdot \vec{S}_1 \vec{S}_1 \cdot \vec{v}_2 \right) + \\
 & \frac{1}{r^5} \left( \frac{529}{4} \left( \hat{n} \cdot \vec{v}_1 \right)^2 \left( \hat{n} \cdot \vec{S}_1 \right)^2 - \frac{803}{4} \hat{n} \cdot \vec{v}_1 \hat{n} \cdot \vec{v}_2 \left( \hat{n} \cdot \vec{S}_1 \right)^2 - \frac{7}{4} \vec{v}_1 \cdot \vec{v}_1 \left( \hat{n} \cdot \vec{S}_1 \right)^2 + \frac{45}{4} \vec{v}_1 \cdot \vec{v}_2 \left( \hat{n} \cdot \vec{S}_1 \right)^2 - \right. \\
 & \left. 67 \hat{n} \cdot \vec{v}_1 \vec{S}_1 \cdot \vec{v}_1 \hat{n} \cdot \vec{S}_1 + \frac{57}{2} \hat{n} \cdot \vec{v}_2 \vec{S}_1 \cdot \vec{v}_1 \hat{n} \cdot \vec{S}_1 + \frac{157}{2} \hat{n} \cdot \vec{v}_1 \vec{S}_1 \cdot \vec{v}_2 \hat{n} \cdot \vec{S}_1 + \frac{3}{2} \left( \vec{S}_1 \cdot \vec{v}_1 \right)^2 - \right. \\
 & \left. \frac{7}{4} \left( \hat{n} \cdot \vec{v}_1 \right)^2 \vec{S}_1 \cdot \vec{S}_1 + \frac{93}{4} \hat{n} \cdot \vec{v}_1 \hat{n} \cdot \vec{v}_2 \vec{S}_1 \cdot \vec{S}_1 - \frac{13}{2} \vec{S}_1 \cdot \vec{v}_1 \vec{S}_1 \cdot \vec{v}_2 - \frac{5}{4} \vec{S}_1 \cdot \vec{S}_1 \vec{v}_1 \cdot \vec{v}_1 - \frac{17}{4} \vec{S}_1 \cdot \vec{S}_1 \vec{v}_1 \cdot \vec{v}_2 \right) + \\
 & \left. \pi^2 \left( \frac{-\frac{3}{2} \left( \hat{n} \cdot \vec{S}_1 \right)^2 - \frac{3}{2} \hat{n} \cdot \vec{S}_1 \hat{n} \cdot \vec{S}_1 + \frac{1}{2} \vec{S}_1 \cdot \vec{S}_1 + \frac{1}{2} \vec{S}_1 \cdot \vec{S}_1}{r^3} + \frac{1}{r^4} \right. \right. \\
 & \left( \frac{15}{8} \hat{n} \cdot \vec{a}_1 \left( \hat{n} \cdot \vec{S}_1 \right)^2 + \frac{15}{2} \hat{n} \cdot \vec{S}_1 \hat{n} \cdot \vec{v}_1 \hat{n} \cdot \vec{S}_1 - \frac{15}{2} \hat{n} \cdot \vec{S}_1 \hat{n} \cdot \vec{v}_2 \hat{n} \cdot \vec{S}_1 - \frac{3}{2} \vec{S}_1 \cdot \vec{v}_1 \hat{n} \cdot \vec{S}_1 + \frac{3}{2} \vec{S}_1 \cdot \vec{v}_2 \hat{n} \cdot \vec{S}_1 - \right. \\
 & \left. \frac{3}{4} \vec{S}_1 \cdot \vec{a}_1 \hat{n} \cdot \vec{S}_1 - \frac{3}{2} \hat{n} \cdot \vec{v}_1 \vec{S}_1 \cdot \vec{S}_1 + \frac{3}{2} \hat{n} \cdot \vec{v}_2 \vec{S}_1 \cdot \vec{S}_1 - \frac{3}{8} \hat{n} \cdot \vec{a}_1 \vec{S}_1 \cdot \vec{S}_1 - \frac{3}{2} \hat{n} \cdot \vec{S}_1 \vec{S}_1 \cdot \vec{v}_1 + \frac{3}{2} \hat{n} \cdot \vec{S}_1 \vec{S}_1 \cdot \vec{v}_2 \right) + \frac{1}{r^5} \\
 & \left( -\frac{525}{64} \left( \hat{n} \cdot \vec{v}_1 \right)^2 \left( \hat{n} \cdot \vec{S}_1 \right)^2 + \frac{1155}{64} \hat{n} \cdot \vec{v}_1 \hat{n} \cdot \vec{v}_2 \left( \hat{n} \cdot \vec{S}_1 \right)^2 + \frac{75}{64} \vec{v}_1 \cdot \vec{v}_1 \left( \hat{n} \cdot \vec{S}_1 \right)^2 - \frac{165}{64} \vec{v}_1 \cdot \vec{v}_2 \left( \hat{n} \cdot \vec{S}_1 \right)^2 + \right. \\
 & \left. \frac{75}{16} \hat{n} \cdot \vec{v}_1 \vec{S}_1 \cdot \vec{v}_1 \hat{n} \cdot \vec{S}_1 - \frac{165}{32} \hat{n} \cdot \vec{v}_2 \vec{S}_1 \cdot \vec{v}_1 \hat{n} \cdot \vec{S}_1 - \frac{165}{32} \hat{n} \cdot \vec{v}_1 \vec{S}_1 \cdot \vec{v}_2 \hat{n} \cdot \vec{S}_1 - \frac{15}{32} \left( \vec{S}_1 \cdot \vec{v}_1 \right)^2 + \frac{75}{64} \left( \hat{n} \cdot \vec{v}_1 \right)^2 \right. \\
 & \left. \left. \left. \vec{S}_1 \cdot \vec{S}_1 - \frac{165}{64} \hat{n} \cdot \vec{v}_1 \hat{n} \cdot \vec{v}_2 \vec{S}_1 \cdot \vec{S}_1 + \frac{33}{32} \vec{S}_1 \cdot \vec{v}_1 \vec{S}_1 \cdot \vec{v}_2 - \frac{15}{64} \vec{S}_1 \cdot \vec{S}_1 \vec{v}_1 \cdot \vec{v}_1 + \frac{33}{64} \vec{S}_1 \cdot \vec{S}_1 \vec{v}_1 \cdot \vec{v}_2 \right) \right) \right) m_2^2 C_{ES^2 1} \}
 \end{aligned}$$

{DiagS1CES2[3, 9, 2],

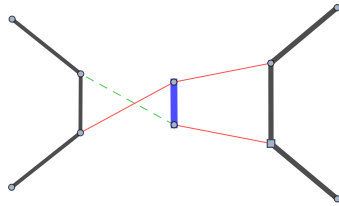

,

$$\begin{aligned}
 G^3 & \left( \frac{1}{r^4} \left( 19 \hat{n} \cdot \vec{a}_2 \left( \hat{n} \cdot \vec{S}_1 \right)^2 + 58 \hat{n} \cdot \vec{S}_1 \hat{n} \cdot \vec{v}_2 \hat{n} \cdot \vec{S}_1 - 2 \vec{S}_1 \cdot \vec{v}_2 \hat{n} \cdot \vec{S}_1 - \right. \right. \\
 & \left. \left. 2 \vec{S}_1 \cdot \vec{a}_2 \hat{n} \cdot \vec{S}_1 - 2 \hat{n} \cdot \vec{v}_2 \vec{S}_1 \cdot \vec{S}_1 - 3 \hat{n} \cdot \vec{a}_2 \vec{S}_1 \cdot \vec{S}_1 - 2 \hat{n} \cdot \vec{S}_1 \vec{S}_1 \cdot \vec{v}_2 \right) + \frac{1}{r^5} \right.
 \end{aligned}$$

$$\begin{aligned}
& \left( \frac{803}{4} (\hat{n} \cdot \vec{v}_2)^2 (\hat{n} \cdot \vec{S}_1)^2 - \frac{529}{4} \hat{n} \cdot \vec{v}_1 \hat{n} \cdot \vec{v}_2 (\hat{n} \cdot \vec{S}_1)^2 + \frac{7}{4} \vec{v}_1 \cdot \vec{v}_2 (\hat{n} \cdot \vec{S}_1)^2 - \frac{45}{4} \vec{v}_2 \cdot \vec{v}_2 (\hat{n} \cdot \vec{S}_1)^2 + \right. \\
& \frac{127}{2} \hat{n} \cdot \vec{v}_2 \vec{S}_1 \cdot \vec{v}_1 \hat{n} \cdot \vec{S}_1 + \frac{7}{2} \hat{n} \cdot \vec{v}_1 \vec{S}_1 \cdot \vec{v}_2 \hat{n} \cdot \vec{S}_1 - 107 \hat{n} \cdot \vec{v}_2 \vec{S}_1 \cdot \vec{v}_2 \hat{n} \cdot \vec{S}_1 + \frac{13}{2} (\vec{S}_1 \cdot \vec{v}_2)^2 - \frac{93}{4} (\hat{n} \cdot \vec{v}_2)^2 \vec{S}_1 \cdot \vec{S}_1 + \\
& \frac{7}{4} \hat{n} \cdot \vec{v}_1 \hat{n} \cdot \vec{v}_2 \vec{S}_1 \cdot \vec{S}_1 - \frac{3}{2} \vec{S}_1 \cdot \vec{v}_1 \vec{S}_1 \cdot \vec{v}_2 + \frac{5}{4} \vec{S}_1 \cdot \vec{S}_1 \vec{v}_1 \cdot \vec{v}_2 + \frac{17}{4} \vec{S}_1 \cdot \vec{S}_1 \vec{v}_2 \cdot \vec{v}_2 \left. \right) + \pi^2 \left( \frac{1}{r^4} \left( -\frac{15}{8} \hat{n} \cdot \vec{a}_2 (\hat{n} \cdot \vec{S}_1)^2 - \right. \right. \\
& \frac{15}{4} \hat{n} \cdot \vec{S}_1 \hat{n} \cdot \vec{v}_2 \hat{n} \cdot \vec{S}_1 + \frac{3}{4} \vec{S}_1 \cdot \vec{v}_2 \hat{n} \cdot \vec{S}_1 + \frac{3}{4} \vec{S}_1 \cdot \vec{a}_2 \hat{n} \cdot \vec{S}_1 + \frac{3}{4} \hat{n} \cdot \vec{v}_2 \vec{S}_1 \cdot \vec{S}_1 + \frac{3}{8} \hat{n} \cdot \vec{a}_2 \vec{S}_1 \cdot \vec{S}_1 + \frac{3}{4} \hat{n} \cdot \vec{S}_1 \vec{S}_1 \cdot \vec{v}_2 \left. \right) + \\
& \frac{1}{r^5} \left( -\frac{1155}{64} (\hat{n} \cdot \vec{v}_2)^2 (\hat{n} \cdot \vec{S}_1)^2 + \frac{525}{64} \hat{n} \cdot \vec{v}_1 \hat{n} \cdot \vec{v}_2 (\hat{n} \cdot \vec{S}_1)^2 - \frac{75}{64} \vec{v}_1 \cdot \vec{v}_2 (\hat{n} \cdot \vec{S}_1)^2 + \frac{165}{64} \vec{v}_2 \cdot \vec{v}_2 (\hat{n} \cdot \vec{S}_1)^2 - \right. \\
& \frac{75}{32} \hat{n} \cdot \vec{v}_2 \vec{S}_1 \cdot \vec{v}_1 \hat{n} \cdot \vec{S}_1 - \frac{75}{32} \hat{n} \cdot \vec{v}_1 \vec{S}_1 \cdot \vec{v}_2 \hat{n} \cdot \vec{S}_1 + \frac{165}{16} \hat{n} \cdot \vec{v}_2 \vec{S}_1 \cdot \vec{v}_2 \hat{n} \cdot \vec{S}_1 - \frac{33}{32} (\vec{S}_1 \cdot \vec{v}_2)^2 + \frac{165}{64} (\hat{n} \cdot \vec{v}_2)^2 \\
& \left. \left. \vec{S}_1 \cdot \vec{S}_1 - \frac{75}{64} \hat{n} \cdot \vec{v}_1 \hat{n} \cdot \vec{v}_2 \vec{S}_1 \cdot \vec{S}_1 + \frac{15}{32} \vec{S}_1 \cdot \vec{v}_1 \vec{S}_1 \cdot \vec{v}_2 + \frac{15}{64} \vec{S}_1 \cdot \vec{S}_1 \vec{v}_1 \cdot \vec{v}_2 - \frac{33}{64} \vec{S}_1 \cdot \vec{S}_1 \vec{v}_2 \cdot \vec{v}_2 \right) \right) \left. \right) m_2^2 C_{ES^2 1} \}
\end{aligned}$$

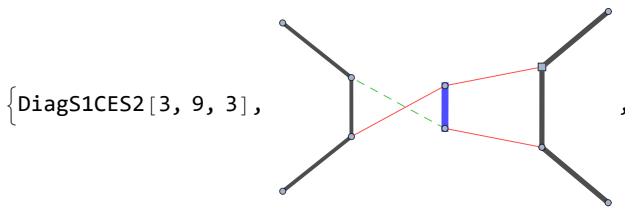

$$\begin{aligned}
& G^3 m_2^2 C_{ES^2 1} \left( \frac{189 \hat{n} \cdot \vec{a}_2 (\hat{n} \cdot \vec{S}_1)^2 - 78 \vec{S}_1 \cdot \vec{a}_2 \hat{n} \cdot \vec{S}_1 - 29 \vec{S}_1 \cdot \vec{S}_1 \hat{n} \cdot \vec{a}_2}{r^4} + \right. \\
& \pi^2 \left( \frac{-\frac{75}{8} \hat{n} \cdot \vec{a}_2 (\hat{n} \cdot \vec{S}_1)^2 + \frac{15}{4} \vec{S}_1 \cdot \vec{a}_2 \hat{n} \cdot \vec{S}_1 + \frac{15}{8} \vec{S}_1 \cdot \vec{S}_1 \hat{n} \cdot \vec{a}_2}{r^4} + \frac{1}{r^5} \left( \frac{525}{64} (\hat{n} \cdot \vec{S}_1)^2 (\hat{n} \cdot \vec{v}_2)^2 + \right. \right. \\
& \frac{525}{64} (\hat{n} \cdot \vec{S}_1)^2 \hat{n} \cdot \vec{v}_1 \hat{n} \cdot \vec{v}_2 - \frac{75}{64} \vec{v}_1 \cdot \vec{v}_2 (\hat{n} \cdot \vec{S}_1)^2 - \frac{75}{64} \vec{v}_2 \cdot \vec{v}_2 (\hat{n} \cdot \vec{S}_1)^2 - \frac{75}{32} \hat{n} \cdot \vec{S}_1 \hat{n} \cdot \vec{v}_2 \vec{S}_1 \cdot \vec{v}_1 - \\
& \frac{75}{32} \hat{n} \cdot \vec{S}_1 \hat{n} \cdot \vec{v}_1 \vec{S}_1 \cdot \vec{v}_2 - \frac{75}{16} \hat{n} \cdot \vec{S}_1 \hat{n} \cdot \vec{v}_2 \vec{S}_1 \cdot \vec{v}_2 - \frac{75}{64} \vec{S}_1 \cdot \vec{S}_1 (\hat{n} \cdot \vec{v}_2)^2 - \frac{75}{64} \vec{S}_1 \cdot \vec{S}_1 \hat{n} \cdot \vec{v}_1 \hat{n} \cdot \vec{v}_2 + \\
& \left. \left. \frac{15}{32} (\vec{S}_1 \cdot \vec{v}_2)^2 + \frac{15}{32} \vec{S}_1 \cdot \vec{v}_1 \vec{S}_1 \cdot \vec{v}_2 + \frac{15}{64} \vec{S}_1 \cdot \vec{S}_1 \vec{v}_1 \cdot \vec{v}_2 + \frac{15}{64} \vec{S}_1 \cdot \vec{S}_1 \vec{v}_2 \cdot \vec{v}_2 \right) \right) + \frac{1}{r^5} \\
& \left( -\frac{9}{4} (\hat{n} \cdot \vec{S}_1)^2 (\hat{n} \cdot \vec{v}_2)^2 - \frac{445}{4} (\hat{n} \cdot \vec{S}_1)^2 \hat{n} \cdot \vec{v}_1 \hat{n} \cdot \vec{v}_2 + \frac{27}{4} \vec{v}_1 \cdot \vec{v}_2 (\hat{n} \cdot \vec{S}_1)^2 + \frac{55}{4} \vec{v}_2 \cdot \vec{v}_2 (\hat{n} \cdot \vec{S}_1)^2 - \right. \\
& \frac{29}{2} \hat{n} \cdot \vec{S}_1 \hat{n} \cdot \vec{v}_2 \vec{S}_1 \cdot \vec{v}_1 + \frac{91}{2} \hat{n} \cdot \vec{S}_1 \hat{n} \cdot \vec{v}_1 \vec{S}_1 \cdot \vec{v}_2 + 21 \hat{n} \cdot \vec{S}_1 \hat{n} \cdot \vec{v}_2 \vec{S}_1 \cdot \vec{v}_2 - \frac{25}{4} \vec{S}_1 \cdot \vec{S}_1 (\hat{n} \cdot \vec{v}_2)^2 + \\
& \left. \left. \frac{91}{4} \vec{S}_1 \cdot \vec{S}_1 \hat{n} \cdot \vec{v}_1 \hat{n} \cdot \vec{v}_2 - \frac{15}{2} (\vec{S}_1 \cdot \vec{v}_2)^2 + \frac{9}{2} \vec{S}_1 \cdot \vec{v}_1 \vec{S}_1 \cdot \vec{v}_2 - \frac{31}{4} \vec{S}_1 \cdot \vec{S}_1 \vec{v}_1 \cdot \vec{v}_2 + \frac{13}{4} \vec{S}_1 \cdot \vec{S}_1 \vec{v}_2 \cdot \vec{v}_2 \right) \right) \}
\end{aligned}$$

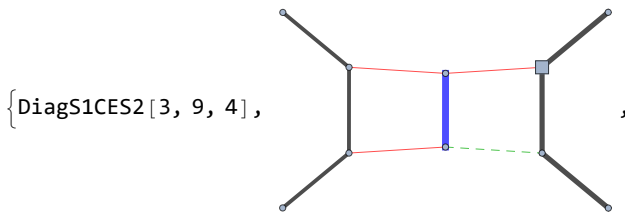

$$G^3 m_2^2 C_{ES^2 1} \left( \frac{-159 \hat{n} \cdot \vec{a}_1 (\hat{n} \cdot \vec{S}_1)^2 + 70 \vec{S}_1 \cdot \vec{a}_1 \hat{n} \cdot \vec{S}_1 + 11 \vec{S}_1 \cdot \vec{S}_1 \hat{n} \cdot \vec{a}_1}{r^4} + \right.$$

$$\pi^2 \left( \frac{\frac{75}{8} \hat{n} \cdot \vec{a}_1 (\hat{n} \cdot \vec{S}_1)^2 - \frac{15}{4} \vec{S}_1 \cdot \vec{a}_1 \hat{n} \cdot \vec{S}_1 - \frac{15}{8} \vec{S}_1 \cdot \vec{S}_1 \hat{n} \cdot \vec{a}_1}{r^4} + \frac{1}{r^5} \left( -\frac{525}{64} (\hat{n} \cdot \vec{S}_1)^2 (\hat{n} \cdot \vec{v}_1)^2 - \right. \right. \\ \left. \frac{525}{64} (\hat{n} \cdot \vec{S}_1)^2 \hat{n} \cdot \vec{v}_1 \hat{n} \cdot \vec{v}_2 + \frac{75}{64} \vec{v}_1 \cdot \vec{v}_1 (\hat{n} \cdot \vec{S}_1)^2 + \frac{75}{64} \vec{v}_1 \cdot \vec{v}_2 (\hat{n} \cdot \vec{S}_1)^2 + \frac{75}{16} \hat{n} \cdot \vec{S}_1 \hat{n} \cdot \vec{v}_1 \vec{S}_1 \cdot \vec{v}_1 + \right. \\ \left. \frac{75}{32} \hat{n} \cdot \vec{S}_1 \hat{n} \cdot \vec{v}_2 \vec{S}_1 \cdot \vec{v}_1 + \frac{75}{32} \hat{n} \cdot \vec{S}_1 \hat{n} \cdot \vec{v}_1 \vec{S}_1 \cdot \vec{v}_2 + \frac{75}{64} \vec{S}_1 \cdot \vec{S}_1 (\hat{n} \cdot \vec{v}_1)^2 + \frac{75}{64} \vec{S}_1 \cdot \vec{S}_1 \hat{n} \cdot \vec{v}_1 \hat{n} \cdot \vec{v}_2 - \right. \\ \left. \frac{15}{32} (\vec{S}_1 \cdot \vec{v}_1)^2 - \frac{15}{32} \vec{S}_1 \cdot \vec{v}_1 \vec{S}_1 \cdot \vec{v}_2 - \frac{15}{64} \vec{S}_1 \cdot \vec{S}_1 \vec{v}_1 \cdot \vec{v}_1 - \frac{15}{64} \vec{S}_1 \cdot \vec{S}_1 \vec{v}_1 \cdot \vec{v}_2 \right) \Bigg) + \frac{1}{r^5} \\ \left( \frac{445}{4} (\hat{n} \cdot \vec{S}_1)^2 (\hat{n} \cdot \vec{v}_1)^2 + \frac{9}{4} (\hat{n} \cdot \vec{S}_1)^2 \hat{n} \cdot \vec{v}_1 \hat{n} \cdot \vec{v}_2 - \frac{27}{4} \vec{v}_1 \cdot \vec{v}_1 (\hat{n} \cdot \vec{S}_1)^2 - \frac{55}{4} \vec{v}_1 \cdot \vec{v}_2 (\hat{n} \cdot \vec{S}_1)^2 - \right. \\ \left. 31 \hat{n} \cdot \vec{S}_1 \hat{n} \cdot \vec{v}_1 \vec{S}_1 \cdot \vec{v}_1 + \frac{29}{2} \hat{n} \cdot \vec{S}_1 \hat{n} \cdot \vec{v}_2 \vec{S}_1 \cdot \vec{v}_1 - \frac{71}{2} \hat{n} \cdot \vec{S}_1 \hat{n} \cdot \vec{v}_1 \vec{S}_1 \cdot \vec{v}_2 - \frac{91}{4} \vec{S}_1 \cdot \vec{S}_1 (\hat{n} \cdot \vec{v}_1)^2 + \right. \\ \left. \frac{25}{4} \vec{S}_1 \cdot \vec{S}_1 \hat{n} \cdot \vec{v}_1 \hat{n} \cdot \vec{v}_2 - \frac{9}{2} (\vec{S}_1 \cdot \vec{v}_1)^2 + \frac{15}{2} \vec{S}_1 \cdot \vec{v}_1 \vec{S}_1 \cdot \vec{v}_2 + \frac{31}{4} \vec{S}_1 \cdot \vec{S}_1 \vec{v}_1 \cdot \vec{v}_1 - \frac{13}{4} \vec{S}_1 \cdot \vec{S}_1 \vec{v}_1 \cdot \vec{v}_2 \right) \Bigg) \Bigg\}$$

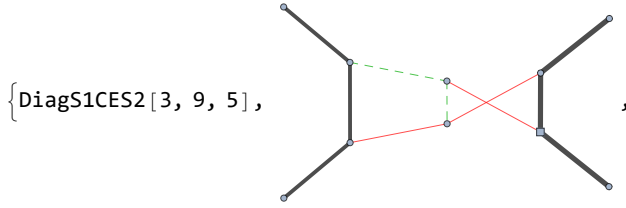

$$G^3 m_2^2 C_{ES^2 1} \left( \frac{1}{r^5} \pi^2 \left( \frac{105}{64} (\hat{n} \cdot \vec{S}_1)^2 (\hat{n} \cdot \vec{v}_2)^2 + \frac{105}{64} (\hat{n} \cdot \vec{S}_1)^2 \hat{n} \cdot \vec{v}_1 \hat{n} \cdot \vec{v}_2 - \frac{15}{64} \vec{v}_1 \cdot \vec{v}_2 (\hat{n} \cdot \vec{S}_1)^2 - \frac{15}{64} \vec{v}_2 \cdot \vec{v}_2 (\hat{n} \cdot \vec{S}_1)^2 - \right. \right. \\ \left. \frac{15}{32} \hat{n} \cdot \vec{S}_1 \hat{n} \cdot \vec{v}_2 \vec{S}_1 \cdot \vec{v}_1 - \frac{15}{32} \hat{n} \cdot \vec{S}_1 \hat{n} \cdot \vec{v}_1 \vec{S}_1 \cdot \vec{v}_2 - \frac{15}{16} \hat{n} \cdot \vec{S}_1 \hat{n} \cdot \vec{v}_2 \vec{S}_1 \cdot \vec{v}_2 - \frac{15}{64} \vec{S}_1 \cdot \vec{S}_1 (\hat{n} \cdot \vec{v}_2)^2 - \right. \\ \left. \frac{15}{64} \vec{S}_1 \cdot \vec{S}_1 \hat{n} \cdot \vec{v}_1 \hat{n} \cdot \vec{v}_2 + \frac{3}{32} (\vec{S}_1 \cdot \vec{v}_2)^2 + \frac{3}{32} \vec{S}_1 \cdot \vec{v}_1 \vec{S}_1 \cdot \vec{v}_2 + \frac{3}{64} \vec{S}_1 \cdot \vec{S}_1 \vec{v}_1 \cdot \vec{v}_2 + \frac{3}{64} \vec{S}_1 \cdot \vec{S}_1 \vec{v}_2 \cdot \vec{v}_2 \right) + \\ \frac{1}{r^5} \left( -\frac{101}{4} (\hat{n} \cdot \vec{S}_1)^2 (\hat{n} \cdot \vec{v}_2)^2 - \frac{13}{4} (\hat{n} \cdot \vec{S}_1)^2 \hat{n} \cdot \vec{v}_1 \hat{n} \cdot \vec{v}_2 + \frac{27}{4} \vec{v}_1 \cdot \vec{v}_2 (\hat{n} \cdot \vec{S}_1)^2 - \frac{21}{4} \vec{v}_2 \cdot \vec{v}_2 (\hat{n} \cdot \vec{S}_1)^2 + \right. \\ \left. \frac{3}{2} \hat{n} \cdot \vec{S}_1 \hat{n} \cdot \vec{v}_2 \vec{S}_1 \cdot \vec{v}_1 - \frac{13}{2} \hat{n} \cdot \vec{S}_1 \hat{n} \cdot \vec{v}_1 \vec{S}_1 \cdot \vec{v}_2 + 9 \hat{n} \cdot \vec{S}_1 \hat{n} \cdot \vec{v}_2 \vec{S}_1 \cdot \vec{v}_2 + \frac{43}{4} \vec{S}_1 \cdot \vec{S}_1 (\hat{n} \cdot \vec{v}_2)^2 + \right. \\ \left. \frac{27}{4} \vec{S}_1 \cdot \vec{S}_1 \hat{n} \cdot \vec{v}_1 \hat{n} \cdot \vec{v}_2 - \frac{3}{2} (\vec{S}_1 \cdot \vec{v}_2)^2 + \frac{1}{2} \vec{S}_1 \cdot \vec{v}_1 \vec{S}_1 \cdot \vec{v}_2 - \frac{15}{4} \vec{S}_1 \cdot \vec{S}_1 \vec{v}_1 \cdot \vec{v}_2 + \frac{9}{4} \vec{S}_1 \cdot \vec{S}_1 \vec{v}_2 \cdot \vec{v}_2 \right) \Bigg) \Bigg\}$$

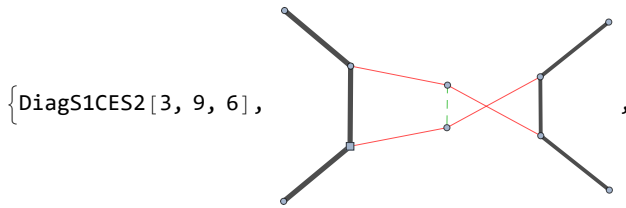

$$G^3 \left( \frac{1}{r^4} \left( -\frac{5}{2} \hat{n} \cdot \vec{S}_1 \hat{n} \cdot \vec{S}_1 \hat{n} \cdot \vec{v}_1 + \frac{1}{2} \vec{S}_1 \cdot \vec{S}_1 \hat{n} \cdot \vec{v}_1 + 2 \hat{n} \cdot \vec{S}_1 \hat{n} \cdot \vec{S}_1 \hat{n} \cdot \vec{v}_2 - \right. \right. \\ \left. \frac{3}{2} \hat{n} \cdot \vec{S}_1 \vec{S}_1 \cdot \vec{v}_1 - \frac{3}{2} \hat{n} \cdot \vec{S}_1 \vec{S}_1 \cdot \vec{v}_2 - \hat{n} \cdot \vec{v}_2 \vec{S}_1 \cdot \vec{S}_1 - \frac{3}{2} \hat{n} \cdot \vec{S}_1 \vec{S}_1 \cdot \vec{v}_1 - \frac{3}{2} \hat{n} \cdot \vec{S}_1 \vec{S}_1 \cdot \vec{v}_2 \right) + \frac{1}{r^5} \\ \left( \frac{11}{2} (\hat{n} \cdot \vec{v}_1)^2 (\hat{n} \cdot \vec{S}_1)^2 - \frac{1}{8} (\hat{n} \cdot \vec{v}_2)^2 (\hat{n} \cdot \vec{S}_1)^2 - \frac{1}{8} \hat{n} \cdot \vec{v}_1 \hat{n} \cdot \vec{v}_2 (\hat{n} \cdot \vec{S}_1)^2 + \frac{5}{2} \vec{v}_1 \cdot \vec{v}_1 (\hat{n} \cdot \vec{S}_1)^2 + \right. \\ \left. \frac{27}{8} \vec{v}_1 \cdot \vec{v}_2 (\hat{n} \cdot \vec{S}_1)^2 + \frac{31}{8} \vec{v}_2 \cdot \vec{v}_2 (\hat{n} \cdot \vec{S}_1)^2 + \frac{11}{4} \hat{n} \cdot \vec{v}_2 \vec{S}_1 \cdot \vec{v}_1 \hat{n} \cdot \vec{S}_1 + \frac{9}{4} \hat{n} \cdot \vec{v}_1 \vec{S}_1 \cdot \vec{v}_2 \hat{n} \cdot \vec{S}_1 + \frac{3}{2} \hat{n} \cdot \vec{v}_2 \vec{S}_1 \cdot \vec{v}_2 \hat{n} \cdot \vec{S}_1 - \right. \\ \left. \frac{1}{2} \vec{S}_1 \cdot \vec{S}_1 (\hat{n} \cdot \vec{v}_1)^2 - \frac{1}{2} \vec{S}_1 \cdot \vec{S}_1 \hat{n} \cdot \vec{v}_1 \hat{n} \cdot \vec{v}_2 + \frac{1}{4} \vec{S}_1 \cdot \vec{S}_1 \vec{v}_1 \cdot \vec{v}_1 + \frac{1}{4} \vec{S}_1 \cdot \vec{S}_1 \vec{v}_1 \cdot \vec{v}_2 + \frac{1}{4} \vec{S}_1 \cdot \vec{S}_1 \vec{v}_2 \cdot \vec{v}_2 \right) \Bigg) \Bigg\}$$



$$\begin{aligned}
 & \left( \vec{S}_1 \cdot \vec{v}_1 \right)^2 - \frac{3}{4} \left( \vec{S}_1 \cdot \vec{v}_2 \right)^2 - \frac{1}{2} \left( \hat{n} \cdot \vec{v}_1 \right)^2 \vec{S}_1 \cdot \vec{S}_1 - \frac{9}{8} \left( \hat{n} \cdot \vec{v}_2 \right)^2 \vec{S}_1 \cdot \vec{S}_1 - \frac{5}{8} \hat{n} \cdot \vec{v}_1 \hat{n} \cdot \vec{v}_2 \vec{S}_1 \cdot \vec{S}_1 - \\
 & \frac{9}{4} \vec{S}_1 \cdot \vec{v}_1 \vec{S}_1 \cdot \vec{v}_2 - \frac{1}{2} \vec{S}_1 \cdot \vec{S}_1 \vec{v}_1 \cdot \vec{v}_1 + \frac{5}{8} \vec{S}_1 \cdot \vec{S}_1 \vec{v}_1 \cdot \vec{v}_2 - \frac{3}{8} \vec{S}_1 \cdot \vec{S}_1 \vec{v}_2 \cdot \vec{v}_2 \Big) + \\
 & \pi^2 \left( \frac{-\frac{15}{32} \hat{n} \cdot \vec{S}_1 \hat{n} \cdot \vec{S}_1 \hat{n} \cdot \vec{v}_2 + \frac{3}{32} \vec{S}_1 \cdot \vec{S}_1 \hat{n} \cdot \vec{v}_2 + \frac{3}{32} \hat{n} \cdot \vec{S}_1 \vec{S}_1 \cdot \vec{v}_2 + \frac{3}{32} \hat{n} \cdot \vec{S}_1 \vec{S}_1 \cdot \vec{v}_2}{r^4} + \frac{1}{r^5} \right. \\
 & \left( \frac{105}{128} \left( \hat{n} \cdot \vec{v}_2 \right)^2 \left( \hat{n} \cdot \vec{S}_1 \right)^2 + \frac{105}{128} \hat{n} \cdot \vec{v}_1 \hat{n} \cdot \vec{v}_2 \left( \hat{n} \cdot \vec{S}_1 \right)^2 - \frac{15}{128} \vec{v}_1 \cdot \vec{v}_2 \left( \hat{n} \cdot \vec{S}_1 \right)^2 - \frac{15}{128} \vec{v}_2 \cdot \vec{v}_2 \left( \hat{n} \cdot \vec{S}_1 \right)^2 - \right. \\
 & \frac{15}{64} \hat{n} \cdot \vec{v}_2 \vec{S}_1 \cdot \vec{v}_1 \hat{n} \cdot \vec{S}_1 - \frac{15}{64} \hat{n} \cdot \vec{v}_1 \vec{S}_1 \cdot \vec{v}_2 \hat{n} \cdot \vec{S}_1 - \frac{15}{32} \hat{n} \cdot \vec{v}_2 \vec{S}_1 \cdot \vec{v}_2 \hat{n} \cdot \vec{S}_1 + \frac{3}{64} \left( \vec{S}_1 \cdot \vec{v}_2 \right)^2 - \frac{15}{128} \left( \hat{n} \cdot \vec{v}_2 \right)^2 \\
 & \left. \left. \left. \vec{S}_1 \cdot \vec{S}_1 - \frac{15}{128} \hat{n} \cdot \vec{v}_1 \hat{n} \cdot \vec{v}_2 \vec{S}_1 \cdot \vec{S}_1 + \frac{3}{64} \vec{S}_1 \cdot \vec{v}_1 \vec{S}_1 \cdot \vec{v}_2 + \frac{3}{128} \vec{S}_1 \cdot \vec{S}_1 \vec{v}_1 \cdot \vec{v}_2 + \frac{3}{128} \vec{S}_1 \cdot \vec{S}_1 \vec{v}_2 \cdot \vec{v}_2 \right) \right) \right) m_2^2 C_{ES^2 1} \Big\}
 \end{aligned}$$

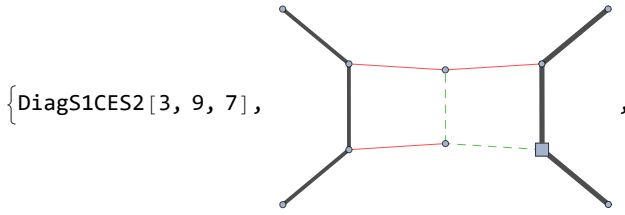

$$\begin{aligned}
 & G^3 \left( \frac{-10 \hat{n} \cdot \vec{S}_1 \hat{n} \cdot \vec{S}_1 \hat{n} \cdot \vec{v}_2 + 14 \vec{S}_1 \cdot \vec{S}_1 \hat{n} \cdot \vec{v}_2 + 2 \hat{n} \cdot \vec{S}_1 \vec{S}_1 \cdot \vec{v}_1 + 4 \hat{n} \cdot \vec{v}_1 \vec{S}_1 \cdot \vec{S}_1 + 2 \hat{n} \cdot \vec{S}_1 \vec{S}_1 \cdot \vec{v}_1}{r^4} + \frac{1}{r^5} \right. \\
 & \left( \frac{13}{4} \left( \hat{n} \cdot \vec{v}_1 \right)^2 \left( \hat{n} \cdot \vec{S}_1 \right)^2 + \frac{101}{4} \hat{n} \cdot \vec{v}_1 \hat{n} \cdot \vec{v}_2 \left( \hat{n} \cdot \vec{S}_1 \right)^2 - \frac{27}{4} \vec{v}_1 \cdot \vec{v}_1 \left( \hat{n} \cdot \vec{S}_1 \right)^2 + \frac{21}{4} \vec{v}_1 \cdot \vec{v}_2 \left( \hat{n} \cdot \vec{S}_1 \right)^2 + \right. \\
 & 5 \hat{n} \cdot \vec{v}_1 \vec{S}_1 \cdot \vec{v}_1 \hat{n} \cdot \vec{S}_1 + \frac{1}{2} \hat{n} \cdot \vec{v}_2 \vec{S}_1 \cdot \vec{v}_1 \hat{n} \cdot \vec{S}_1 - \frac{19}{2} \hat{n} \cdot \vec{v}_1 \vec{S}_1 \cdot \vec{v}_2 \hat{n} \cdot \vec{S}_1 - \frac{1}{2} \left( \vec{S}_1 \cdot \vec{v}_1 \right)^2 - \\
 & \frac{27}{4} \left( \hat{n} \cdot \vec{v}_1 \right)^2 \vec{S}_1 \cdot \vec{S}_1 - \frac{43}{4} \hat{n} \cdot \vec{v}_1 \hat{n} \cdot \vec{v}_2 \vec{S}_1 \cdot \vec{S}_1 + \frac{3}{2} \vec{S}_1 \cdot \vec{v}_1 \vec{S}_1 \cdot \vec{v}_2 + \frac{15}{4} \vec{S}_1 \cdot \vec{S}_1 \vec{v}_1 \cdot \vec{v}_1 - \frac{9}{4} \vec{S}_1 \cdot \vec{S}_1 \vec{v}_1 \cdot \vec{v}_2 \Big) + \\
 & \pi^2 \left( \frac{1}{r^4} \left( \frac{15}{4} \hat{n} \cdot \vec{S}_1 \hat{n} \cdot \vec{S}_1 \hat{n} \cdot \vec{v}_1 - \frac{3}{4} \vec{S}_1 \cdot \vec{S}_1 \hat{n} \cdot \vec{v}_1 + \frac{15}{4} \hat{n} \cdot \vec{S}_1 \hat{n} \cdot \vec{S}_1 \hat{n} \cdot \vec{v}_2 - \frac{3}{4} \hat{n} \cdot \vec{S}_1 \vec{S}_1 \cdot \vec{v}_1 - \right. \right. \\
 & \left. \frac{3}{4} \hat{n} \cdot \vec{S}_1 \vec{S}_1 \cdot \vec{v}_2 - \frac{3}{4} \hat{n} \cdot \vec{v}_2 \vec{S}_1 \cdot \vec{S}_1 - \frac{3}{4} \hat{n} \cdot \vec{S}_1 \vec{S}_1 \cdot \vec{v}_1 - \frac{3}{4} \hat{n} \cdot \vec{S}_1 \vec{S}_1 \cdot \vec{v}_2 \right) + \frac{1}{r^5} \\
 & \left( -\frac{525}{64} \left( \hat{n} \cdot \vec{v}_1 \right)^2 \left( \hat{n} \cdot \vec{S}_1 \right)^2 - \frac{525}{64} \hat{n} \cdot \vec{v}_1 \hat{n} \cdot \vec{v}_2 \left( \hat{n} \cdot \vec{S}_1 \right)^2 + \frac{75}{64} \vec{v}_1 \cdot \vec{v}_1 \left( \hat{n} \cdot \vec{S}_1 \right)^2 + \frac{75}{64} \vec{v}_1 \cdot \vec{v}_2 \left( \hat{n} \cdot \vec{S}_1 \right)^2 + \right. \\
 & \frac{75}{16} \hat{n} \cdot \vec{v}_1 \vec{S}_1 \cdot \vec{v}_1 \hat{n} \cdot \vec{S}_1 + \frac{75}{32} \hat{n} \cdot \vec{v}_2 \vec{S}_1 \cdot \vec{v}_1 \hat{n} \cdot \vec{S}_1 + \frac{75}{32} \hat{n} \cdot \vec{v}_1 \vec{S}_1 \cdot \vec{v}_2 \hat{n} \cdot \vec{S}_1 - \frac{15}{32} \left( \vec{S}_1 \cdot \vec{v}_1 \right)^2 + \frac{75}{64} \left( \hat{n} \cdot \vec{v}_1 \right)^2 \vec{S}_1 \cdot \vec{S}_1 + \\
 & \left. \left. \left. \frac{75}{64} \hat{n} \cdot \vec{v}_1 \hat{n} \cdot \vec{v}_2 \vec{S}_1 \cdot \vec{S}_1 - \frac{15}{32} \vec{S}_1 \cdot \vec{v}_1 \vec{S}_1 \cdot \vec{v}_2 - \frac{15}{64} \vec{S}_1 \cdot \vec{S}_1 \vec{v}_1 \cdot \vec{v}_1 - \frac{15}{64} \vec{S}_1 \cdot \vec{S}_1 \vec{v}_1 \cdot \vec{v}_2 \right) \right) \right) m_2^2 C_{ES^2 1} \Big\}
 \end{aligned}$$

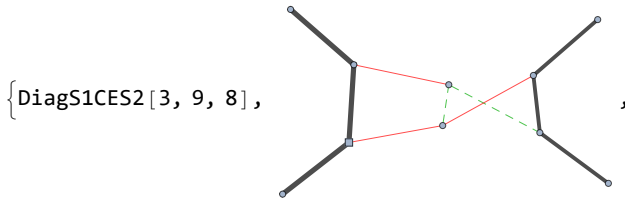

$$\begin{aligned}
& G^3 \left( \frac{-10 \hat{n} \cdot \vec{S}_1 \hat{n} \cdot \vec{S}_1 \hat{n} \cdot \vec{v}_2 + 10 \vec{S}_1 \cdot \vec{S}_1 \hat{n} \cdot \vec{v}_2 - 2 \hat{n} \cdot \vec{S}_1 \vec{S}_1 \cdot \vec{v}_2 - 2 \hat{n} \cdot \vec{S}_1 \vec{S}_1 \cdot \vec{v}_2}{r^4} + \frac{1}{r^5} \right. \\
& \left( \frac{39}{4} (\hat{n} \cdot \vec{v}_2)^2 (\hat{n} \cdot \vec{S}_1)^2 + \frac{127}{4} \hat{n} \cdot \vec{v}_1 \hat{n} \cdot \vec{v}_2 (\hat{n} \cdot \vec{S}_1)^2 + \frac{7}{4} \vec{v}_1 \cdot \vec{v}_2 (\hat{n} \cdot \vec{S}_1)^2 - \frac{41}{4} \vec{v}_2 \cdot \vec{v}_2 (\hat{n} \cdot \vec{S}_1)^2 - \right. \\
& \frac{17}{2} \hat{n} \cdot \vec{v}_2 \vec{S}_1 \cdot \vec{v}_1 \hat{n} \cdot \vec{S}_1 + \frac{7}{2} \hat{n} \cdot \vec{v}_1 \vec{S}_1 \cdot \vec{v}_2 \hat{n} \cdot \vec{S}_1 + 9 \hat{n} \cdot \vec{v}_2 \vec{S}_1 \cdot \vec{v}_2 \hat{n} \cdot \vec{S}_1 - \frac{7}{2} (\vec{S}_1 \cdot \vec{v}_2)^2 - \\
& \frac{57}{4} (\hat{n} \cdot \vec{v}_2)^2 \vec{S}_1 \cdot \vec{S}_1 - \frac{73}{4} \hat{n} \cdot \vec{v}_1 \hat{n} \cdot \vec{v}_2 \vec{S}_1 \cdot \vec{S}_1 - \frac{3}{2} \vec{S}_1 \cdot \vec{v}_1 \vec{S}_1 \cdot \vec{v}_2 + \frac{5}{4} \vec{S}_1 \cdot \vec{S}_1 \vec{v}_1 \cdot \vec{v}_2 + \frac{29}{4} \vec{S}_1 \cdot \vec{S}_1 \vec{v}_2 \cdot \vec{v}_2 \Big) + \\
& \left. \pi^2 \left( \frac{\frac{15}{2} \hat{n} \cdot \vec{S}_1 \hat{n} \cdot \vec{S}_1 \hat{n} \cdot \vec{v}_2 - \frac{3}{2} \vec{S}_1 \cdot \vec{S}_1 \hat{n} \cdot \vec{v}_2 - \frac{3}{2} \hat{n} \cdot \vec{S}_1 \vec{S}_1 \cdot \vec{v}_2 - \frac{3}{2} \hat{n} \cdot \vec{S}_1 \vec{S}_1 \cdot \vec{v}_2}{r^4} + \frac{1}{r^5} \right. \right. \\
& \left( -\frac{1575}{64} (\hat{n} \cdot \vec{v}_2)^2 (\hat{n} \cdot \vec{S}_1)^2 - \frac{1575}{64} \hat{n} \cdot \vec{v}_1 \hat{n} \cdot \vec{v}_2 (\hat{n} \cdot \vec{S}_1)^2 + \frac{225}{64} \vec{v}_1 \cdot \vec{v}_2 (\hat{n} \cdot \vec{S}_1)^2 + \frac{225}{64} \vec{v}_2 \cdot \vec{v}_2 (\hat{n} \cdot \vec{S}_1)^2 + \right. \\
& \frac{225}{32} \hat{n} \cdot \vec{v}_2 \vec{S}_1 \cdot \vec{v}_1 \hat{n} \cdot \vec{S}_1 + \frac{225}{32} \hat{n} \cdot \vec{v}_1 \vec{S}_1 \cdot \vec{v}_2 \hat{n} \cdot \vec{S}_1 + \frac{225}{16} \hat{n} \cdot \vec{v}_2 \vec{S}_1 \cdot \vec{v}_2 \hat{n} \cdot \vec{S}_1 - \frac{45}{32} (\vec{S}_1 \cdot \vec{v}_2)^2 + \frac{225}{64} (\hat{n} \cdot \vec{v}_2)^2 \\
& \left. \left. \left. \vec{S}_1 \cdot \vec{S}_1 + \frac{225}{64} \hat{n} \cdot \vec{v}_1 \hat{n} \cdot \vec{v}_2 \vec{S}_1 \cdot \vec{S}_1 - \frac{45}{32} \vec{S}_1 \cdot \vec{v}_1 \vec{S}_1 \cdot \vec{v}_2 - \frac{45}{64} \vec{S}_1 \cdot \vec{S}_1 \vec{v}_1 \cdot \vec{v}_2 - \frac{45}{64} \vec{S}_1 \cdot \vec{S}_1 \vec{v}_2 \cdot \vec{v}_2 \right) \right) \right) m_2^2 C_{ES^2_1} \Big\}
\end{aligned}$$

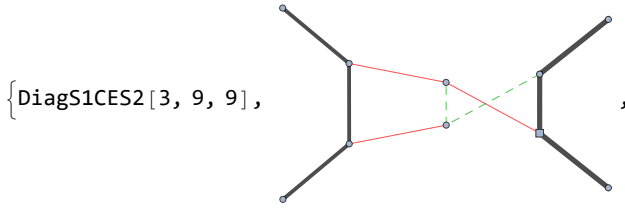

$$\begin{aligned}
& G^3 \left( \frac{10 \hat{n} \cdot \vec{S}_1 \hat{n} \cdot \vec{S}_1 \hat{n} \cdot \vec{v}_1 - 10 \vec{S}_1 \cdot \vec{S}_1 \hat{n} \cdot \vec{v}_1 + 2 \hat{n} \cdot \vec{S}_1 \vec{S}_1 \cdot \vec{v}_1 + 2 \hat{n} \cdot \vec{S}_1 \vec{S}_1 \cdot \vec{v}_1}{r^4} + \frac{1}{r^5} \right. \\
& \left( -\frac{127}{4} (\hat{n} \cdot \vec{v}_1)^2 (\hat{n} \cdot \vec{S}_1)^2 - \frac{39}{4} \hat{n} \cdot \vec{v}_1 \hat{n} \cdot \vec{v}_2 (\hat{n} \cdot \vec{S}_1)^2 - \frac{7}{4} \vec{v}_1 \cdot \vec{v}_1 (\hat{n} \cdot \vec{S}_1)^2 + \frac{41}{4} \vec{v}_1 \cdot \vec{v}_2 (\hat{n} \cdot \vec{S}_1)^2 + \right. \\
& 5 \hat{n} \cdot \vec{v}_1 \vec{S}_1 \cdot \vec{v}_1 \hat{n} \cdot \vec{S}_1 - \frac{19}{2} \hat{n} \cdot \vec{v}_2 \vec{S}_1 \cdot \vec{v}_1 \hat{n} \cdot \vec{S}_1 + \frac{1}{2} \hat{n} \cdot \vec{v}_1 \vec{S}_1 \cdot \vec{v}_2 \hat{n} \cdot \vec{S}_1 + \frac{3}{2} (\vec{S}_1 \cdot \vec{v}_1)^2 + \\
& \frac{73}{4} (\hat{n} \cdot \vec{v}_1)^2 \vec{S}_1 \cdot \vec{S}_1 + \frac{57}{4} \hat{n} \cdot \vec{v}_1 \hat{n} \cdot \vec{v}_2 \vec{S}_1 \cdot \vec{S}_1 + \frac{7}{2} \vec{S}_1 \cdot \vec{v}_1 \vec{S}_1 \cdot \vec{v}_2 - \frac{5}{4} \vec{S}_1 \cdot \vec{S}_1 \vec{v}_1 \cdot \vec{v}_1 - \frac{29}{4} \vec{S}_1 \cdot \vec{S}_1 \vec{v}_1 \cdot \vec{v}_2 \Big) + \\
& \left. \pi^2 \left( \frac{\frac{15}{4} \hat{n} \cdot \vec{S}_1 \hat{n} \cdot \vec{S}_1 \hat{n} \cdot \vec{v}_1 - \frac{3}{4} \vec{S}_1 \cdot \vec{S}_1 \hat{n} \cdot \vec{v}_1 - \frac{3}{4} \hat{n} \cdot \vec{S}_1 \vec{S}_1 \cdot \vec{v}_1 - \frac{3}{4} \hat{n} \cdot \vec{S}_1 \vec{S}_1 \cdot \vec{v}_1}{r^4} + \frac{1}{r^5} \right. \right. \\
& \left( -\frac{525}{64} (\hat{n} \cdot \vec{v}_1)^2 (\hat{n} \cdot \vec{S}_1)^2 - \frac{525}{64} \hat{n} \cdot \vec{v}_1 \hat{n} \cdot \vec{v}_2 (\hat{n} \cdot \vec{S}_1)^2 + \frac{75}{64} \vec{v}_1 \cdot \vec{v}_1 (\hat{n} \cdot \vec{S}_1)^2 + \frac{75}{64} \vec{v}_1 \cdot \vec{v}_2 (\hat{n} \cdot \vec{S}_1)^2 + \right. \\
& \frac{75}{16} \hat{n} \cdot \vec{v}_1 \vec{S}_1 \cdot \vec{v}_1 \hat{n} \cdot \vec{S}_1 + \frac{75}{32} \hat{n} \cdot \vec{v}_2 \vec{S}_1 \cdot \vec{v}_1 \hat{n} \cdot \vec{S}_1 + \frac{75}{32} \hat{n} \cdot \vec{v}_1 \vec{S}_1 \cdot \vec{v}_2 \hat{n} \cdot \vec{S}_1 - \frac{15}{32} (\vec{S}_1 \cdot \vec{v}_1)^2 + \frac{75}{64} (\hat{n} \cdot \vec{v}_1)^2 \vec{S}_1 \cdot \vec{S}_1 + \\
& \left. \left. \left. \frac{75}{64} \hat{n} \cdot \vec{v}_1 \hat{n} \cdot \vec{v}_2 \vec{S}_1 \cdot \vec{S}_1 - \frac{15}{32} \vec{S}_1 \cdot \vec{v}_1 \vec{S}_1 \cdot \vec{v}_2 - \frac{15}{64} \vec{S}_1 \cdot \vec{S}_1 \vec{v}_1 \cdot \vec{v}_1 - \frac{15}{64} \vec{S}_1 \cdot \vec{S}_1 \vec{v}_1 \cdot \vec{v}_2 \right) \right) \right) m_2^2 C_{ES^2_1} \Big\}
\end{aligned}$$

{DiagS1CES2[3, 9, 10],

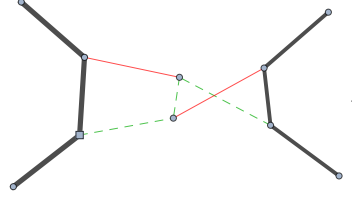

,

$$G^3 m_2^2 C_{ES^2 1} \left( \frac{1}{r^5} \left( -88 \left( \hat{n} \cdot \vec{S}_1 \right)^2 \hat{n} \cdot \vec{v}_1 \hat{n} \cdot \vec{v}_2 + 40 \vec{v}_1 \cdot \vec{v}_2 \left( \hat{n} \cdot \vec{S}_1 \right)^2 + 8 \hat{n} \cdot \vec{S}_1 \hat{n} \cdot \vec{v}_2 \vec{S}_1 \cdot \vec{v}_1 + 48 \hat{n} \cdot \vec{S}_1 \hat{n} \cdot \vec{v}_1 \vec{S}_1 \cdot \vec{v}_2 + 16 \vec{S}_1 \cdot \vec{S}_1 \right. \right. \\ \left. \left. \hat{n} \cdot \vec{v}_1 \hat{n} \cdot \vec{v}_2 - 8 \vec{S}_1 \cdot \vec{v}_1 \vec{S}_1 \cdot \vec{v}_2 - 16 \vec{S}_1 \cdot \vec{S}_1 \vec{v}_1 \cdot \vec{v}_2 \right) + \frac{40 \hat{n} \cdot \vec{S}_1 \hat{n} \cdot \vec{S}_1 \hat{n} \cdot \vec{v}_2 - 20 \hat{n} \cdot \vec{S}_1 \vec{S}_1 \cdot \vec{v}_2 - 20 \hat{n} \cdot \vec{S}_1 \vec{S}_1 \cdot \vec{v}_2}{r^4} \right) \}$$

{DiagS1CES2[3, 9, 11],

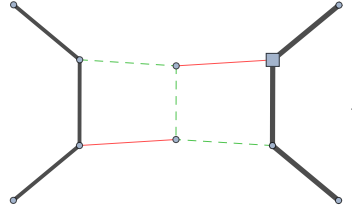

,  $\frac{1}{r^5}$

$$G^3 m_2^2 C_{ES^2 1} \left( -88 \left( \hat{n} \cdot \vec{S}_1 \right)^2 \hat{n} \cdot \vec{v}_1 \hat{n} \cdot \vec{v}_2 + 40 \vec{v}_1 \cdot \vec{v}_2 \left( \hat{n} \cdot \vec{S}_1 \right)^2 + 48 \hat{n} \cdot \vec{S}_1 \hat{n} \cdot \vec{v}_2 \vec{S}_1 \cdot \vec{v}_1 + \right. \\ \left. 8 \hat{n} \cdot \vec{S}_1 \hat{n} \cdot \vec{v}_1 \vec{S}_1 \cdot \vec{v}_2 + 16 \vec{S}_1 \cdot \vec{S}_1 \hat{n} \cdot \vec{v}_1 \hat{n} \cdot \vec{v}_2 - 8 \vec{S}_1 \cdot \vec{v}_1 \vec{S}_1 \cdot \vec{v}_2 - 16 \vec{S}_1 \cdot \vec{S}_1 \vec{v}_1 \cdot \vec{v}_2 \right) \}$$

{DiagS1CES2[3, 9, 12],

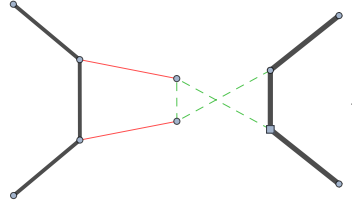

,

$$G^3 m_2^2 C_{ES^2 1} \left( \frac{1}{r^5} \left( 88 \left( \hat{n} \cdot \vec{S}_1 \right)^2 \left( \hat{n} \cdot \vec{v}_1 \right)^2 - 40 \vec{v}_1 \cdot \vec{v}_1 \left( \hat{n} \cdot \vec{S}_1 \right)^2 - 56 \hat{n} \cdot \vec{S}_1 \hat{n} \cdot \vec{v}_1 \vec{S}_1 \cdot \vec{v}_1 - 16 \vec{S}_1 \cdot \vec{S}_1 \left( \hat{n} \cdot \vec{v}_1 \right)^2 + \right. \right. \\ \left. \left. 8 \left( \vec{S}_1 \cdot \vec{v}_1 \right)^2 + 16 \vec{S}_1 \cdot \vec{S}_1 \vec{v}_1 \cdot \vec{v}_1 \right) + \frac{-40 \hat{n} \cdot \vec{S}_1 \hat{n} \cdot \vec{S}_1 \hat{n} \cdot \vec{v}_1 + 20 \hat{n} \cdot \vec{S}_1 \vec{S}_1 \cdot \vec{v}_1 + 20 \hat{n} \cdot \vec{S}_1 \vec{S}_1 \cdot \vec{v}_1}{r^4} \right) \}$$

{DiagS1CES2[3, 9, 13],

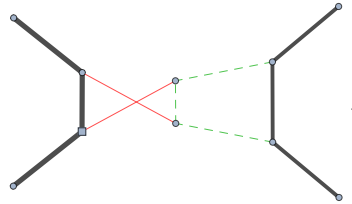

,  $\frac{1}{r^5}$

$$G^3 m_2^2 C_{ES^2 1} \left( 88 \left( \hat{n} \cdot \vec{S}_1 \right)^2 \left( \hat{n} \cdot \vec{v}_2 \right)^2 - 40 \vec{v}_2 \cdot \vec{v}_2 \left( \hat{n} \cdot \vec{S}_1 \right)^2 - 56 \hat{n} \cdot \vec{S}_1 \hat{n} \cdot \vec{v}_2 \vec{S}_1 \cdot \vec{v}_2 - \right. \\ \left. 16 \vec{S}_1 \cdot \vec{S}_1 \left( \hat{n} \cdot \vec{v}_2 \right)^2 + 8 \left( \vec{S}_1 \cdot \vec{v}_2 \right)^2 + 16 \vec{S}_1 \cdot \vec{S}_1 \vec{v}_2 \cdot \vec{v}_2 \right) \}$$

{DiagS1CES2[3, 9, 14],

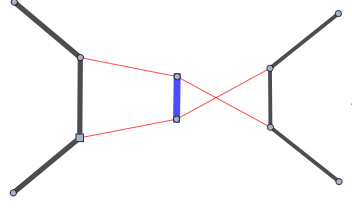

,

$$\begin{aligned}
 G^3 m_2^2 C_{ES^2 1} & \left( \frac{1}{r^4} \left( 6 \vec{S}_1 \cdot \vec{a}_1 \hat{n} \cdot \vec{S}_1 - 14 \hat{n} \cdot \vec{S}_1 \hat{n} \cdot \vec{S}_1 \hat{n} \cdot \vec{v}_2 + \vec{S}_1 \cdot \vec{S}_1 \hat{n} \cdot \vec{v}_2 + \right. \right. \\
 & 6 \hat{n} \cdot \vec{S}_1 \vec{S}_1 \cdot \vec{v}_1 + \frac{7}{2} \hat{n} \cdot \vec{S}_1 \vec{S}_1 \cdot \vec{v}_2 - 12 \vec{S}_1 \cdot \vec{S}_1 \hat{n} \cdot \vec{v}_1 + 6 \hat{n} \cdot \vec{S}_1 \vec{S}_1 \cdot \vec{v}_1 + \frac{7}{2} \hat{n} \cdot \vec{S}_1 \vec{S}_1 \cdot \vec{v}_2 \Big) + \\
 & \frac{1}{r^5} \left( 50 \left( \hat{n} \cdot \vec{S}_1 \right)^2 \hat{n} \cdot \vec{v}_1 \hat{n} \cdot \vec{v}_2 - 45 \vec{v}_1 \cdot \vec{v}_1 \left( \hat{n} \cdot \vec{S}_1 \right)^2 - \frac{21}{2} \vec{v}_1 \cdot \vec{v}_2 \left( \hat{n} \cdot \vec{S}_1 \right)^2 - 45 \vec{v}_2 \cdot \vec{v}_2 \left( \hat{n} \cdot \vec{S}_1 \right)^2 + \right. \\
 & 15 \hat{n} \cdot \vec{S}_1 \hat{n} \cdot \vec{v}_1 \vec{S}_1 \cdot \vec{v}_1 - 15 \hat{n} \cdot \vec{S}_1 \hat{n} \cdot \vec{v}_2 \vec{S}_1 \cdot \vec{v}_1 - \frac{29}{2} \hat{n} \cdot \vec{S}_1 \hat{n} \cdot \vec{v}_1 \vec{S}_1 \cdot \vec{v}_2 - 15 \vec{S}_1 \cdot \vec{S}_1 \left( \hat{n} \cdot \vec{v}_1 \right)^2 - \frac{9}{2} \vec{S}_1 \cdot \vec{S}_1 \hat{n} \cdot \vec{v}_1 \hat{n} \cdot \vec{v}_2 - \\
 & 7 \left( \vec{S}_1 \cdot \vec{v}_1 \right)^2 + \frac{7}{2} \vec{S}_1 \cdot \vec{v}_1 \vec{S}_1 \cdot \vec{v}_2 + 10 \vec{S}_1 \cdot \vec{S}_1 \vec{v}_1 \cdot \vec{v}_1 + 2 \vec{S}_1 \cdot \vec{S}_1 \vec{v}_1 \cdot \vec{v}_2 + 3 \vec{S}_1 \cdot \vec{S}_1 \vec{v}_2 \cdot \vec{v}_2 \Big) + \\
 & \pi^2 \left( \frac{1}{r^5} \left( -\frac{315}{64} \left( \hat{n} \cdot \vec{S}_1 \right)^2 \hat{n} \cdot \vec{v}_1 \hat{n} \cdot \vec{v}_2 + \frac{45}{64} \vec{v}_1 \cdot \vec{v}_2 \left( \hat{n} \cdot \vec{S}_1 \right)^2 + \frac{45}{32} \hat{n} \cdot \vec{S}_1 \hat{n} \cdot \vec{v}_2 \vec{S}_1 \cdot \vec{v}_1 + \right. \right. \\
 & \frac{45}{32} \hat{n} \cdot \vec{S}_1 \hat{n} \cdot \vec{v}_1 \vec{S}_1 \cdot \vec{v}_2 + \frac{45}{64} \vec{S}_1 \cdot \vec{S}_1 \hat{n} \cdot \vec{v}_1 \hat{n} \cdot \vec{v}_2 - \frac{9}{32} \vec{S}_1 \cdot \vec{v}_1 \vec{S}_1 \cdot \vec{v}_2 - \frac{9}{64} \vec{S}_1 \cdot \vec{S}_1 \vec{v}_1 \cdot \vec{v}_2 \Big) + \\
 & \left. \left. \frac{45}{32} \hat{n} \cdot \vec{S}_1 \hat{n} \cdot \vec{S}_1 \hat{n} \cdot \vec{v}_2 - \frac{9}{32} \vec{S}_1 \cdot \vec{S}_1 \hat{n} \cdot \vec{v}_2 - \frac{9}{32} \hat{n} \cdot \vec{S}_1 \vec{S}_1 \cdot \vec{v}_2 - \frac{9}{32} \hat{n} \cdot \vec{S}_1 \vec{S}_1 \cdot \vec{v}_2 \right) \right) + \frac{4 \vec{S}_1^2}{r^3} \Bigg\}
 \end{aligned}$$

{DiagS1CES2[3, 9, 15],

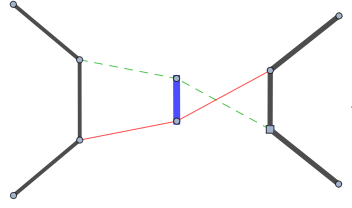

,

$$\begin{aligned}
 G^3 m_2^2 C_{ES^2 1} & \left( \frac{1}{r^5} \left( -88 \left( \hat{n} \cdot \vec{S}_1 \right)^2 \hat{n} \cdot \vec{v}_1 \hat{n} \cdot \vec{v}_2 + 92 \vec{v}_1 \cdot \vec{v}_2 \left( \hat{n} \cdot \vec{S}_1 \right)^2 + 4 \hat{n} \cdot \vec{S}_1 \hat{n} \cdot \vec{v}_2 \vec{S}_1 \cdot \vec{v}_1 + \right. \right. \\
 & 32 \hat{n} \cdot \vec{S}_1 \hat{n} \cdot \vec{v}_1 \vec{S}_1 \cdot \vec{v}_2 + 20 \vec{S}_1 \cdot \vec{S}_1 \hat{n} \cdot \vec{v}_1 \hat{n} \cdot \vec{v}_2 - 4 \vec{S}_1 \cdot \vec{v}_1 \vec{S}_1 \cdot \vec{v}_2 - 16 \vec{S}_1 \cdot \vec{S}_1 \vec{v}_1 \cdot \vec{v}_2 \Big) + \\
 & \left. \frac{48 \hat{n} \cdot \vec{S}_1 \hat{n} \cdot \vec{S}_1 \hat{n} \cdot \vec{v}_2 + 8 \vec{S}_1 \cdot \vec{S}_1 \hat{n} \cdot \vec{v}_2 - 28 \hat{n} \cdot \vec{S}_1 \vec{S}_1 \cdot \vec{v}_2 - 28 \hat{n} \cdot \vec{S}_1 \vec{S}_1 \cdot \vec{v}_2}{r^4} + \right. \\
 & \pi^2 \left( \frac{1}{r^5} \left( \frac{105}{16} \left( \hat{n} \cdot \vec{S}_1 \right)^2 \hat{n} \cdot \vec{v}_1 \hat{n} \cdot \vec{v}_2 - \frac{15}{16} \vec{v}_1 \cdot \vec{v}_2 \left( \hat{n} \cdot \vec{S}_1 \right)^2 - \frac{15}{8} \hat{n} \cdot \vec{S}_1 \hat{n} \cdot \vec{v}_2 \vec{S}_1 \cdot \vec{v}_1 - \right. \right. \\
 & \frac{15}{8} \hat{n} \cdot \vec{S}_1 \hat{n} \cdot \vec{v}_1 \vec{S}_1 \cdot \vec{v}_2 - \frac{15}{16} \vec{S}_1 \cdot \vec{S}_1 \hat{n} \cdot \vec{v}_1 \hat{n} \cdot \vec{v}_2 + \frac{3}{8} \vec{S}_1 \cdot \vec{v}_1 \vec{S}_1 \cdot \vec{v}_2 + \frac{3}{16} \vec{S}_1 \cdot \vec{S}_1 \vec{v}_1 \cdot \vec{v}_2 \Big) + \\
 & \left. \left. \frac{-\frac{15}{4} \hat{n} \cdot \vec{S}_1 \hat{n} \cdot \vec{S}_1 \hat{n} \cdot \vec{v}_2 + \frac{3}{4} \vec{S}_1 \cdot \vec{S}_1 \hat{n} \cdot \vec{v}_2 + \frac{3}{4} \hat{n} \cdot \vec{S}_1 \vec{S}_1 \cdot \vec{v}_2 + \frac{3}{4} \hat{n} \cdot \vec{S}_1 \vec{S}_1 \cdot \vec{v}_2}{r^4} \right) \right) \Bigg\}
 \end{aligned}$$

{DiagS1CES2[3, 9, 16],

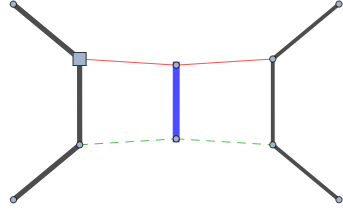

,

$$G^3 m_2^2 C_{ES^2 1} \left( \frac{1}{r^5} \left( -312 \left( \hat{n} \cdot \vec{S}_1 \right)^2 \hat{n} \cdot \vec{v}_1 \hat{n} \cdot \vec{v}_2 + 112 \vec{v}_1 \cdot \vec{v}_2 \left( \hat{n} \cdot \vec{S}_1 \right)^2 + 116 \hat{n} \cdot \vec{S}_1 \hat{n} \cdot \vec{v}_2 \vec{S}_1 \cdot \vec{v}_1 + \right. \right. \\ \left. \left. 84 \hat{n} \cdot \vec{S}_1 \hat{n} \cdot \vec{v}_1 \vec{S}_1 \cdot \vec{v}_2 + 16 \vec{S}_1 \cdot \vec{S}_1 \hat{n} \cdot \vec{v}_1 \hat{n} \cdot \vec{v}_2 - 24 \vec{S}_1 \cdot \vec{v}_1 \vec{S}_1 \cdot \vec{v}_2 - 8 \vec{S}_1 \cdot \vec{S}_1 \vec{v}_1 \cdot \vec{v}_2 \right) + \right. \\ \left. \frac{1}{r^5} \pi^2 \left( \frac{525}{16} \left( \hat{n} \cdot \vec{S}_1 \right)^2 \hat{n} \cdot \vec{v}_1 \hat{n} \cdot \vec{v}_2 - \frac{75}{16} \vec{v}_1 \cdot \vec{v}_2 \left( \hat{n} \cdot \vec{S}_1 \right)^2 - \frac{75}{8} \hat{n} \cdot \vec{S}_1 \hat{n} \cdot \vec{v}_2 \vec{S}_1 \cdot \vec{v}_1 - \right. \right. \\ \left. \left. \frac{75}{8} \hat{n} \cdot \vec{S}_1 \hat{n} \cdot \vec{v}_1 \vec{S}_1 \cdot \vec{v}_2 - \frac{75}{16} \vec{S}_1 \cdot \vec{S}_1 \hat{n} \cdot \vec{v}_1 \hat{n} \cdot \vec{v}_2 + \frac{15}{8} \vec{S}_1 \cdot \vec{v}_1 \vec{S}_1 \cdot \vec{v}_2 + \frac{15}{16} \vec{S}_1 \cdot \vec{S}_1 \vec{v}_1 \cdot \vec{v}_2 \right) \right) \Bigg\}$$

{DiagS1CES2[3, 9, 17],

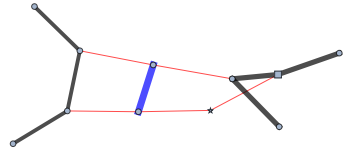

,

$$G^3 \left( \frac{1}{r^4} \left( -\frac{17}{3} \hat{n} \cdot \vec{S}_1 \hat{n} \cdot \vec{S}_1 \hat{n} \cdot \vec{v}_1 + \frac{13}{3} \vec{S}_1 \cdot \vec{S}_1 \hat{n} \cdot \vec{v}_1 + 15 \hat{n} \cdot \vec{S}_1 \hat{n} \cdot \vec{S}_1 \hat{n} \cdot \vec{v}_2 + \right. \right. \\ \left. \left. \frac{7}{3} \hat{n} \cdot \vec{S}_1 \vec{S}_1 \cdot \vec{v}_1 - 3 \hat{n} \cdot \vec{S}_1 \vec{S}_1 \cdot \vec{v}_2 - 11 \hat{n} \cdot \vec{v}_2 \vec{S}_1 \cdot \vec{S}_1 + \frac{7}{3} \hat{n} \cdot \vec{S}_1 \vec{S}_1 \cdot \vec{v}_1 - 3 \hat{n} \cdot \vec{S}_1 \vec{S}_1 \cdot \vec{v}_2 \right) + \frac{1}{r^5} \right. \\ \left( \frac{19}{2} \left( \hat{n} \cdot \vec{v}_1 \right)^2 \left( \hat{n} \cdot \vec{S}_1 \right)^2 - \frac{98}{3} \hat{n} \cdot \vec{v}_1 \hat{n} \cdot \vec{v}_2 \left( \hat{n} \cdot \vec{S}_1 \right)^2 - \frac{7}{2} \vec{v}_1 \cdot \vec{v}_1 \left( \hat{n} \cdot \vec{S}_1 \right)^2 + \frac{14}{3} \vec{v}_1 \cdot \vec{v}_2 \left( \hat{n} \cdot \vec{S}_1 \right)^2 - \right. \\ \left. 8 \hat{n} \cdot \vec{v}_1 \vec{S}_1 \cdot \vec{v}_1 \hat{n} \cdot \vec{S}_1 + \frac{10}{3} \hat{n} \cdot \vec{v}_2 \vec{S}_1 \cdot \vec{v}_1 \hat{n} \cdot \vec{S}_1 + \frac{28}{3} \hat{n} \cdot \vec{v}_1 \vec{S}_1 \cdot \vec{v}_2 \hat{n} \cdot \vec{S}_1 + 3 \left( \vec{S}_1 \cdot \vec{v}_1 \right)^2 - \right. \\ \left. \frac{1}{2} \left( \hat{n} \cdot \vec{v}_1 \right)^2 \vec{S}_1 \cdot \vec{S}_1 + \frac{50}{3} \hat{n} \cdot \vec{v}_1 \hat{n} \cdot \vec{v}_2 \vec{S}_1 \cdot \vec{S}_1 - \frac{2}{3} \vec{S}_1 \cdot \vec{v}_1 \vec{S}_1 \cdot \vec{v}_2 - \frac{5}{2} \vec{S}_1 \cdot \vec{S}_1 \vec{v}_1 \cdot \vec{v}_1 - \frac{10}{3} \vec{S}_1 \cdot \vec{S}_1 \vec{v}_1 \cdot \vec{v}_2 \right) + \\ \pi^2 \left( \frac{1}{r^4} \left( \frac{15}{32} \hat{n} \cdot \vec{S}_1 \hat{n} \cdot \vec{S}_1 \hat{n} \cdot \vec{v}_1 - \frac{3}{32} \vec{S}_1 \cdot \vec{S}_1 \hat{n} \cdot \vec{v}_1 - \frac{15}{8} \hat{n} \cdot \vec{S}_1 \hat{n} \cdot \vec{S}_1 \hat{n} \cdot \vec{v}_2 - \frac{3}{32} \hat{n} \cdot \vec{S}_1 \vec{S}_1 \cdot \vec{v}_1 + \right. \right. \\ \left. \left. \frac{3}{8} \hat{n} \cdot \vec{S}_1 \vec{S}_1 \cdot \vec{v}_2 + \frac{3}{8} \hat{n} \cdot \vec{v}_2 \vec{S}_1 \cdot \vec{S}_1 - \frac{3}{32} \hat{n} \cdot \vec{S}_1 \vec{S}_1 \cdot \vec{v}_1 + \frac{3}{8} \hat{n} \cdot \vec{S}_1 \vec{S}_1 \cdot \vec{v}_2 \right) + \frac{1}{r^5} \right. \\ \left( -\frac{105}{128} \left( \hat{n} \cdot \vec{v}_1 \right)^2 \left( \hat{n} \cdot \vec{S}_1 \right)^2 + \frac{315}{64} \hat{n} \cdot \vec{v}_1 \hat{n} \cdot \vec{v}_2 \left( \hat{n} \cdot \vec{S}_1 \right)^2 + \frac{15}{128} \vec{v}_1 \cdot \vec{v}_1 \left( \hat{n} \cdot \vec{S}_1 \right)^2 - \frac{45}{64} \vec{v}_1 \cdot \vec{v}_2 \left( \hat{n} \cdot \vec{S}_1 \right)^2 + \right. \\ \left. \frac{15}{32} \hat{n} \cdot \vec{v}_1 \vec{S}_1 \cdot \vec{v}_1 \hat{n} \cdot \vec{S}_1 - \frac{45}{32} \hat{n} \cdot \vec{v}_2 \vec{S}_1 \cdot \vec{v}_1 \hat{n} \cdot \vec{S}_1 - \frac{45}{32} \hat{n} \cdot \vec{v}_1 \vec{S}_1 \cdot \vec{v}_2 \hat{n} \cdot \vec{S}_1 - \frac{3}{64} \left( \vec{S}_1 \cdot \vec{v}_1 \right)^2 + \frac{15}{128} \left( \hat{n} \cdot \vec{v}_1 \right)^2 \right. \\ \left. \left. \vec{S}_1 \cdot \vec{S}_1 - \frac{45}{64} \hat{n} \cdot \vec{v}_1 \hat{n} \cdot \vec{v}_2 \vec{S}_1 \cdot \vec{S}_1 + \frac{9}{32} \vec{S}_1 \cdot \vec{v}_1 \vec{S}_1 \cdot \vec{v}_2 - \frac{3}{128} \vec{S}_1 \cdot \vec{S}_1 \vec{v}_1 \cdot \vec{v}_1 + \frac{9}{64} \vec{S}_1 \cdot \vec{S}_1 \vec{v}_1 \cdot \vec{v}_2 \right) \right) \Bigg) m_2^2 C_{ES^2 1} \Bigg\}$$

{DiagS1CES2[3, 9, 18],

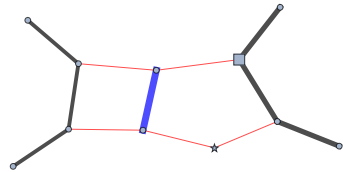

,

$$G^3 \left( \frac{-\frac{73}{3} \hat{n} \cdot \vec{S}_1 \hat{n} \cdot \vec{S}_1 \hat{n} \cdot \vec{v}_1 + \frac{5}{3} \vec{S}_1 \cdot \vec{S}_1 \hat{n} \cdot \vec{v}_1 + \frac{23}{3} \hat{n} \cdot \vec{S}_1 \vec{S}_1 \cdot \vec{v}_1 + \frac{23}{3} \hat{n} \cdot \vec{S}_1 \vec{S}_1 \cdot \vec{v}_1}{r^4} + \frac{1}{r^5} \right. \\ \left( \frac{449}{6} \left( \hat{n} \cdot \vec{v}_1 \right)^2 \left( \hat{n} \cdot \vec{S}_1 \right)^2 - \frac{511}{6} \hat{n} \cdot \vec{v}_1 \hat{n} \cdot \vec{v}_2 \left( \hat{n} \cdot \vec{S}_1 \right)^2 - \frac{101}{6} \vec{v}_1 \cdot \vec{v}_1 \left( \hat{n} \cdot \vec{S}_1 \right)^2 + \frac{73}{6} \vec{v}_1 \cdot \vec{v}_2 \left( \hat{n} \cdot \vec{S}_1 \right)^2 - \right. \\ \left. \left. \frac{15}{32} \hat{n} \cdot \vec{v}_1 \vec{S}_1 \cdot \vec{v}_1 \hat{n} \cdot \vec{S}_1 - \frac{45}{32} \hat{n} \cdot \vec{v}_2 \vec{S}_1 \cdot \vec{v}_1 \hat{n} \cdot \vec{S}_1 - \frac{45}{32} \hat{n} \cdot \vec{v}_1 \vec{S}_1 \cdot \vec{v}_2 \hat{n} \cdot \vec{S}_1 - \frac{3}{64} \left( \vec{S}_1 \cdot \vec{v}_1 \right)^2 + \frac{15}{128} \left( \hat{n} \cdot \vec{v}_1 \right)^2 \right. \right. \\ \left. \left. \vec{S}_1 \cdot \vec{S}_1 - \frac{45}{64} \hat{n} \cdot \vec{v}_1 \hat{n} \cdot \vec{v}_2 \vec{S}_1 \cdot \vec{S}_1 + \frac{9}{32} \vec{S}_1 \cdot \vec{v}_1 \vec{S}_1 \cdot \vec{v}_2 - \frac{3}{128} \vec{S}_1 \cdot \vec{S}_1 \vec{v}_1 \cdot \vec{v}_1 + \frac{9}{64} \vec{S}_1 \cdot \vec{S}_1 \vec{v}_1 \cdot \vec{v}_2 \right) \right) \Bigg) m_2^2 C_{ES^2 1} \Bigg\}$$

$$\begin{aligned}
& \frac{160}{3} \hat{n} \cdot \vec{v}_1 \vec{S}_1 \cdot \vec{v}_1 \hat{n} \cdot \vec{S}_1 + \frac{115}{3} \hat{n} \cdot \vec{v}_2 \vec{S}_1 \cdot \vec{v}_1 \hat{n} \cdot \vec{S}_1 + \frac{73}{3} \hat{n} \cdot \vec{v}_1 \vec{S}_1 \cdot \vec{v}_2 \hat{n} \cdot \vec{S}_1 + \frac{25}{3} (\vec{S}_1 \cdot \vec{v}_1)^2 - \\
& \frac{11}{6} (\hat{n} \cdot \vec{v}_1)^2 \vec{S}_1 \cdot \vec{S}_1 + \frac{25}{6} \hat{n} \cdot \vec{v}_1 \hat{n} \cdot \vec{v}_2 \vec{S}_1 \cdot \vec{S}_1 - \frac{23}{3} \vec{S}_1 \cdot \vec{v}_1 \vec{S}_1 \cdot \vec{v}_2 + \frac{1}{6} \vec{S}_1 \cdot \vec{S}_1 \vec{v}_1 \cdot \vec{v}_1 - \frac{5}{6} \vec{S}_1 \cdot \vec{S}_1 \vec{v}_1 \cdot \vec{v}_2 \Big) + \\
& \pi^2 \left( \frac{\frac{45}{32} \hat{n} \cdot \vec{S}_1 \hat{n} \cdot \vec{S}_1 \hat{n} \cdot \vec{v}_1 - \frac{9}{32} \vec{S}_1 \cdot \vec{S}_1 \hat{n} \cdot \vec{v}_1 - \frac{9}{32} \hat{n} \cdot \vec{S}_1 \vec{S}_1 \cdot \vec{v}_1 - \frac{9}{32} \hat{n} \cdot \vec{S}_1 \vec{S}_1 \cdot \vec{v}_1}{r^4} + \frac{1}{r^5} \right. \\
& \left( -\frac{525}{128} (\hat{n} \cdot \vec{v}_1)^2 (\hat{n} \cdot \vec{S}_1)^2 + \frac{315}{64} \hat{n} \cdot \vec{v}_1 \hat{n} \cdot \vec{v}_2 (\hat{n} \cdot \vec{S}_1)^2 + \frac{75}{128} \vec{v}_1 \cdot \vec{v}_1 (\hat{n} \cdot \vec{S}_1)^2 - \frac{45}{64} \vec{v}_1 \cdot \vec{v}_2 (\hat{n} \cdot \vec{S}_1)^2 + \right. \\
& \frac{75}{32} \hat{n} \cdot \vec{v}_1 \vec{S}_1 \cdot \vec{v}_1 \hat{n} \cdot \vec{S}_1 - \frac{45}{32} \hat{n} \cdot \vec{v}_2 \vec{S}_1 \cdot \vec{v}_1 \hat{n} \cdot \vec{S}_1 - \frac{45}{32} \hat{n} \cdot \vec{v}_1 \vec{S}_1 \cdot \vec{v}_2 \hat{n} \cdot \vec{S}_1 - \frac{15}{64} (\vec{S}_1 \cdot \vec{v}_1)^2 + \frac{75}{128} (\hat{n} \cdot \vec{v}_1)^2 \\
& \left. \left. \vec{S}_1 \cdot \vec{S}_1 - \frac{45}{64} \hat{n} \cdot \vec{v}_1 \hat{n} \cdot \vec{v}_2 \vec{S}_1 \cdot \vec{S}_1 + \frac{9}{32} \vec{S}_1 \cdot \vec{v}_1 \vec{S}_1 \cdot \vec{v}_2 - \frac{15}{128} \vec{S}_1 \cdot \vec{S}_1 \vec{v}_1 \cdot \vec{v}_1 + \frac{9}{64} \vec{S}_1 \cdot \vec{S}_1 \vec{v}_1 \cdot \vec{v}_2 \right) \right) \Bigg] m_{\text{CES}^2 1}^2 \Big\}
\end{aligned}$$

{DiagS1CES2[3, 9, 19],

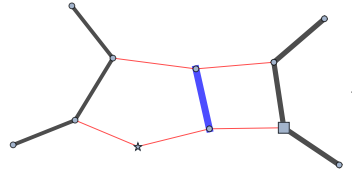

$$\begin{aligned}
& G^3 \left( -\frac{37}{3} \hat{n} \cdot \vec{S}_1 \hat{n} \cdot \vec{S}_1 \hat{n} \cdot \vec{v}_2 + \frac{2}{3} \vec{S}_1 \cdot \vec{S}_1 \hat{n} \cdot \vec{v}_2 + \frac{19}{6} \hat{n} \cdot \vec{S}_1 \vec{S}_1 \cdot \vec{v}_2 + \frac{19}{6} \hat{n} \cdot \vec{S}_1 \vec{S}_1 \cdot \vec{v}_2 \right) + \frac{1}{r^5} \\
& \left( -\frac{323}{12} (\hat{n} \cdot \vec{v}_2)^2 (\hat{n} \cdot \vec{S}_1)^2 + \frac{259}{6} \hat{n} \cdot \vec{v}_1 \hat{n} \cdot \vec{v}_2 (\hat{n} \cdot \vec{S}_1)^2 - \frac{37}{6} \vec{v}_1 \cdot \vec{v}_2 (\hat{n} \cdot \vec{S}_1)^2 + \frac{5}{12} \vec{v}_2 \cdot \vec{v}_2 (\hat{n} \cdot \vec{S}_1)^2 - \right. \\
& \frac{37}{3} \hat{n} \cdot \vec{v}_2 \vec{S}_1 \cdot \vec{v}_1 \hat{n} \cdot \vec{S}_1 - \frac{95}{6} \hat{n} \cdot \vec{v}_1 \vec{S}_1 \cdot \vec{v}_2 \hat{n} \cdot \vec{S}_1 + \frac{85}{6} \hat{n} \cdot \vec{v}_2 \vec{S}_1 \cdot \vec{v}_2 \hat{n} \cdot \vec{S}_1 - \frac{1}{6} (\vec{S}_1 \cdot \vec{v}_2)^2 + \\
& \frac{59}{12} (\hat{n} \cdot \vec{v}_2)^2 \vec{S}_1 \cdot \vec{S}_1 - \frac{5}{3} \hat{n} \cdot \vec{v}_1 \hat{n} \cdot \vec{v}_2 \vec{S}_1 \cdot \vec{S}_1 + \frac{19}{6} \vec{S}_1 \cdot \vec{v}_1 \vec{S}_1 \cdot \vec{v}_2 + \frac{1}{3} \vec{S}_1 \cdot \vec{S}_1 \vec{v}_1 \cdot \vec{v}_2 - \frac{25}{12} \vec{S}_1 \cdot \vec{S}_1 \vec{v}_2 \cdot \vec{v}_2 \Big) + \\
& \pi^2 \left( \frac{\frac{15}{32} \hat{n} \cdot \vec{S}_1 \hat{n} \cdot \vec{S}_1 \hat{n} \cdot \vec{v}_2 - \frac{3}{32} \vec{S}_1 \cdot \vec{S}_1 \hat{n} \cdot \vec{v}_2 - \frac{3}{32} \hat{n} \cdot \vec{S}_1 \vec{S}_1 \cdot \vec{v}_2 - \frac{3}{32} \hat{n} \cdot \vec{S}_1 \vec{S}_1 \cdot \vec{v}_2}{r^4} + \frac{1}{r^5} \right. \\
& \left( \frac{315}{128} (\hat{n} \cdot \vec{v}_2)^2 (\hat{n} \cdot \vec{S}_1)^2 - \frac{105}{64} \hat{n} \cdot \vec{v}_1 \hat{n} \cdot \vec{v}_2 (\hat{n} \cdot \vec{S}_1)^2 + \frac{15}{64} \vec{v}_1 \cdot \vec{v}_2 (\hat{n} \cdot \vec{S}_1)^2 - \frac{45}{128} \vec{v}_2 \cdot \vec{v}_2 (\hat{n} \cdot \vec{S}_1)^2 + \right. \\
& \frac{15}{32} \hat{n} \cdot \vec{v}_2 \vec{S}_1 \cdot \vec{v}_1 \hat{n} \cdot \vec{S}_1 + \frac{15}{32} \hat{n} \cdot \vec{v}_1 \vec{S}_1 \cdot \vec{v}_2 \hat{n} \cdot \vec{S}_1 - \frac{45}{32} \hat{n} \cdot \vec{v}_2 \vec{S}_1 \cdot \vec{v}_2 \hat{n} \cdot \vec{S}_1 + \frac{9}{64} (\vec{S}_1 \cdot \vec{v}_2)^2 - \frac{45}{128} (\hat{n} \cdot \vec{v}_2)^2 \\
& \left. \left. \vec{S}_1 \cdot \vec{S}_1 + \frac{15}{64} \hat{n} \cdot \vec{v}_1 \hat{n} \cdot \vec{v}_2 \vec{S}_1 \cdot \vec{S}_1 - \frac{3}{32} \vec{S}_1 \cdot \vec{v}_1 \vec{S}_1 \cdot \vec{v}_2 - \frac{3}{64} \vec{S}_1 \cdot \vec{S}_1 \vec{v}_1 \cdot \vec{v}_2 + \frac{9}{128} \vec{S}_1 \cdot \vec{S}_1 \vec{v}_2 \cdot \vec{v}_2 \right) \right) \Bigg] m_{\text{CES}^2 1}^2 \Big\}
\end{aligned}$$

{DiagS1CES2[3, 9, 20],

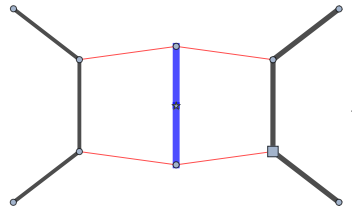

$$\begin{aligned}
G^3 & \left( \frac{1}{r^4} \left( \frac{35}{6} \hat{n} \cdot \vec{S}_1 \hat{n} \cdot \vec{S}_1 \hat{n} \cdot \vec{v}_1 - \frac{7}{6} \vec{S}_1 \cdot \vec{S}_1 \hat{n} \cdot \vec{v}_1 - \frac{70}{3} \hat{n} \cdot \vec{S}_1 \hat{n} \cdot \vec{S}_1 \hat{n} \cdot \vec{v}_2 - \right. \right. \\
& \left. \frac{7}{6} \hat{n} \cdot \vec{S}_1 \vec{S}_1 \cdot \vec{v}_1 + \frac{17}{3} \hat{n} \cdot \vec{S}_1 \vec{S}_1 \cdot \vec{v}_2 + \frac{8}{3} \hat{n} \cdot \vec{v}_2 \vec{S}_1 \cdot \vec{S}_1 - \frac{7}{6} \hat{n} \cdot \vec{S}_1 \vec{S}_1 \cdot \vec{v}_1 + \frac{17}{3} \hat{n} \cdot \vec{S}_1 \vec{S}_1 \cdot \vec{v}_2 \right) + \frac{1}{r^5} \\
& \left( -\frac{35}{2} (\hat{n} \cdot \vec{v}_1)^2 (\hat{n} \cdot \vec{S}_1)^2 - \frac{973}{24} (\hat{n} \cdot \vec{v}_2)^2 (\hat{n} \cdot \vec{S}_1)^2 + \frac{2107}{24} \hat{n} \cdot \vec{v}_1 \hat{n} \cdot \vec{v}_2 (\hat{n} \cdot \vec{S}_1)^2 + \frac{5}{2} \vec{v}_1 \cdot \vec{v}_1 (\hat{n} \cdot \vec{S}_1)^2 - \right. \\
& \frac{421}{24} \vec{v}_1 \cdot \vec{v}_2 (\hat{n} \cdot \vec{S}_1)^2 + \frac{139}{24} \vec{v}_2 \cdot \vec{v}_2 (\hat{n} \cdot \vec{S}_1)^2 + 10 \hat{n} \cdot \vec{v}_1 \vec{S}_1 \cdot \vec{v}_1 \hat{n} \cdot \vec{S}_1 - \frac{301}{12} \hat{n} \cdot \vec{v}_2 \vec{S}_1 \cdot \vec{v}_1 \hat{n} \cdot \vec{S}_1 - \frac{361}{12} \hat{n} \cdot \vec{v}_1 \vec{S}_1 \cdot \vec{v}_2 \\
& \hat{n} \cdot \vec{S}_1 + \frac{169}{6} \hat{n} \cdot \vec{v}_2 \vec{S}_1 \cdot \vec{v}_2 \hat{n} \cdot \vec{S}_1 - (\vec{S}_1 \cdot \vec{v}_1)^2 - \frac{71}{12} (\vec{S}_1 \cdot \vec{v}_2)^2 + \frac{5}{2} (\hat{n} \cdot \vec{v}_1)^2 \vec{S}_1 \cdot \vec{S}_1 + \frac{19}{24} (\hat{n} \cdot \vec{v}_2)^2 \vec{S}_1 \cdot \vec{S}_1 - \\
& \frac{181}{24} \hat{n} \cdot \vec{v}_1 \hat{n} \cdot \vec{v}_2 \vec{S}_1 \cdot \vec{S}_1 + \frac{101}{12} \vec{S}_1 \cdot \vec{v}_1 \vec{S}_1 \cdot \vec{v}_2 - \frac{1}{2} \vec{S}_1 \cdot \vec{S}_1 \vec{v}_1 \cdot \vec{v}_1 - \frac{7}{24} \vec{S}_1 \cdot \vec{S}_1 \vec{v}_1 \cdot \vec{v}_2 + \frac{49}{24} \vec{S}_1 \cdot \vec{S}_1 \vec{v}_2 \cdot \vec{v}_2 \Big) + \\
& \pi^2 \left( \frac{\frac{15}{8} \hat{n} \cdot \vec{S}_1 \hat{n} \cdot \vec{S}_1 \hat{n} \cdot \vec{v}_2 - \frac{3}{8} \vec{S}_1 \cdot \vec{S}_1 \hat{n} \cdot \vec{v}_2 - \frac{3}{8} \hat{n} \cdot \vec{S}_1 \vec{S}_1 \cdot \vec{v}_2 - \frac{3}{8} \hat{n} \cdot \vec{S}_1 \vec{S}_1 \cdot \vec{v}_2}{r^4} + \frac{1}{r^5} \right. \\
& \left( \frac{315}{128} (\hat{n} \cdot \vec{v}_2)^2 (\hat{n} \cdot \vec{S}_1)^2 - \frac{735}{128} \hat{n} \cdot \vec{v}_1 \hat{n} \cdot \vec{v}_2 (\hat{n} \cdot \vec{S}_1)^2 + \frac{105}{128} \vec{v}_1 \cdot \vec{v}_2 (\hat{n} \cdot \vec{S}_1)^2 - \frac{45}{128} \vec{v}_2 \cdot \vec{v}_2 (\hat{n} \cdot \vec{S}_1)^2 + \right. \\
& \frac{105}{64} \hat{n} \cdot \vec{v}_2 \vec{S}_1 \cdot \vec{v}_1 \hat{n} \cdot \vec{S}_1 + \frac{105}{64} \hat{n} \cdot \vec{v}_1 \vec{S}_1 \cdot \vec{v}_2 \hat{n} \cdot \vec{S}_1 - \frac{45}{32} \hat{n} \cdot \vec{v}_2 \vec{S}_1 \cdot \vec{v}_2 \hat{n} \cdot \vec{S}_1 + \frac{9}{64} (\vec{S}_1 \cdot \vec{v}_2)^2 - \frac{45}{128} (\hat{n} \cdot \vec{v}_2)^2 \\
& \left. \left. \vec{S}_1 \cdot \vec{S}_1 + \frac{105}{128} \hat{n} \cdot \vec{v}_1 \hat{n} \cdot \vec{v}_2 \vec{S}_1 \cdot \vec{S}_1 - \frac{21}{64} \vec{S}_1 \cdot \vec{v}_1 \vec{S}_1 \cdot \vec{v}_2 - \frac{21}{128} \vec{S}_1 \cdot \vec{S}_1 \vec{v}_1 \cdot \vec{v}_2 + \frac{9}{128} \vec{S}_1 \cdot \vec{S}_1 \vec{v}_2 \cdot \vec{v}_2 \right) \right) \Bigg\} m_2^2 C_{ES^2 1} \Bigg\}
\end{aligned}$$

{DiagS1CES2[3, 9, 21],

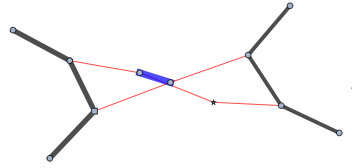

$$\begin{aligned}
G^3 & \left( \frac{\frac{143}{3} \hat{n} \cdot \vec{S}_1 \hat{n} \cdot \vec{S}_1 \hat{n} \cdot \vec{v}_2 - \frac{22}{3} \vec{S}_1 \cdot \vec{S}_1 \hat{n} \cdot \vec{v}_2 - \frac{65}{6} \hat{n} \cdot \vec{S}_1 \vec{S}_1 \cdot \vec{v}_2 - \frac{65}{6} \hat{n} \cdot \vec{S}_1 \vec{S}_1 \cdot \vec{v}_2}{r^4} + \frac{1}{r^5} \right. \\
& \left( \frac{1819}{12} (\hat{n} \cdot \vec{v}_2)^2 (\hat{n} \cdot \vec{S}_1)^2 - \frac{1001}{6} \hat{n} \cdot \vec{v}_1 \hat{n} \cdot \vec{v}_2 (\hat{n} \cdot \vec{S}_1)^2 + \frac{143}{6} \vec{v}_1 \cdot \vec{v}_2 (\hat{n} \cdot \vec{S}_1)^2 - \frac{325}{12} \vec{v}_2 \cdot \vec{v}_2 (\hat{n} \cdot \vec{S}_1)^2 + \right. \\
& \frac{143}{3} \hat{n} \cdot \vec{v}_2 \vec{S}_1 \cdot \vec{v}_1 \hat{n} \cdot \vec{S}_1 + \frac{325}{6} \hat{n} \cdot \vec{v}_1 \vec{S}_1 \cdot \vec{v}_2 \hat{n} \cdot \vec{S}_1 - \frac{551}{6} \hat{n} \cdot \vec{v}_2 \vec{S}_1 \cdot \vec{v}_2 \hat{n} \cdot \vec{S}_1 + \frac{65}{6} (\vec{S}_1 \cdot \vec{v}_2)^2 - \\
& \frac{199}{12} (\hat{n} \cdot \vec{v}_2)^2 \vec{S}_1 \cdot \vec{S}_1 + \frac{55}{3} \hat{n} \cdot \vec{v}_1 \hat{n} \cdot \vec{v}_2 \vec{S}_1 \cdot \vec{S}_1 - \frac{65}{6} \vec{S}_1 \cdot \vec{v}_1 \vec{S}_1 \cdot \vec{v}_2 - \frac{11}{3} \vec{S}_1 \cdot \vec{S}_1 \vec{v}_1 \cdot \vec{v}_2 + \frac{41}{12} \vec{S}_1 \cdot \vec{S}_1 \vec{v}_2 \cdot \vec{v}_2 \Big) + \\
& \pi^2 \left( \frac{-\frac{105}{32} \hat{n} \cdot \vec{S}_1 \hat{n} \cdot \vec{S}_1 \hat{n} \cdot \vec{v}_2 + \frac{21}{32} \vec{S}_1 \cdot \vec{S}_1 \hat{n} \cdot \vec{v}_2 + \frac{21}{32} \hat{n} \cdot \vec{S}_1 \vec{S}_1 \cdot \vec{v}_2 + \frac{21}{32} \hat{n} \cdot \vec{S}_1 \vec{S}_1 \cdot \vec{v}_2}{r^4} + \frac{1}{r^5} \right. \\
& \left( -\frac{1365}{128} (\hat{n} \cdot \vec{v}_2)^2 (\hat{n} \cdot \vec{S}_1)^2 + \frac{735}{64} \hat{n} \cdot \vec{v}_1 \hat{n} \cdot \vec{v}_2 (\hat{n} \cdot \vec{S}_1)^2 - \frac{105}{64} \vec{v}_1 \cdot \vec{v}_2 (\hat{n} \cdot \vec{S}_1)^2 + \frac{195}{128} \vec{v}_2 \cdot \vec{v}_2 (\hat{n} \cdot \vec{S}_1)^2 - \right. \\
& \frac{105}{32} \hat{n} \cdot \vec{v}_2 \vec{S}_1 \cdot \vec{v}_1 \hat{n} \cdot \vec{S}_1 - \frac{105}{32} \hat{n} \cdot \vec{v}_1 \vec{S}_1 \cdot \vec{v}_2 \hat{n} \cdot \vec{S}_1 + \frac{195}{32} \hat{n} \cdot \vec{v}_2 \vec{S}_1 \cdot \vec{v}_2 \hat{n} \cdot \vec{S}_1 - \frac{39}{64} (\vec{S}_1 \cdot \vec{v}_2)^2 + \frac{195}{128} (\hat{n} \cdot \vec{v}_2)^2 \\
& \left. \left. \vec{S}_1 \cdot \vec{S}_1 - \frac{105}{64} \hat{n} \cdot \vec{v}_1 \hat{n} \cdot \vec{v}_2 \vec{S}_1 \cdot \vec{S}_1 + \frac{21}{32} \vec{S}_1 \cdot \vec{v}_1 \vec{S}_1 \cdot \vec{v}_2 + \frac{21}{64} \vec{S}_1 \cdot \vec{S}_1 \vec{v}_1 \cdot \vec{v}_2 - \frac{39}{128} \vec{S}_1 \cdot \vec{S}_1 \vec{v}_2 \cdot \vec{v}_2 \right) \right) \Bigg\} m_2^2 C_{ES^2 1} \Bigg\}
\end{aligned}$$
