# Supplementary material for: N$^3$LO Quadratic-in-Spin Interactions for Generic Compact Binaries
Source: arXiv:2209.09235 ancillary file (2023-01-27)
Supplement: Supplementary file 3 [file graphs-S1S1.pdf]

The diagram results are presented in MS-bar scheme.

Definitions :  $G = G_N$ ,  $\epsilon_d = d - 3$ ,  $\hat{n} = \frac{\vec{x}_1 - \vec{x}_2}{r}$ ,  $\vec{A} = d^j \vec{A} / dt^j$

Legends :

- 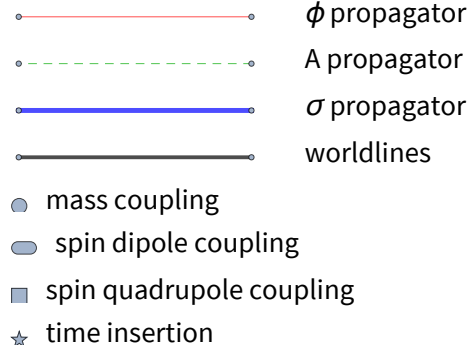  $\phi$  propagator
- 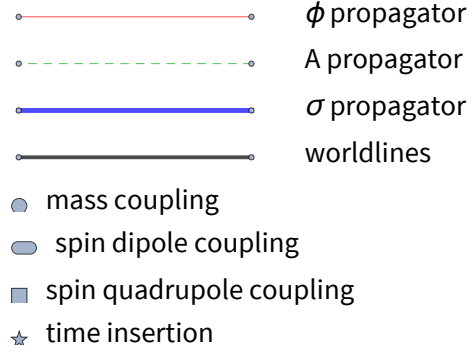 A propagator
- 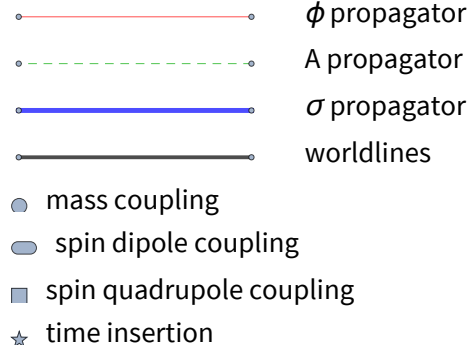  $\sigma$  propagator
- 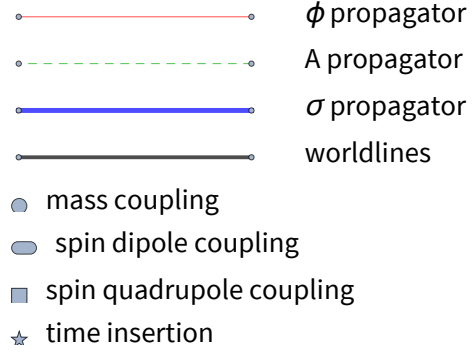 worldlines
- 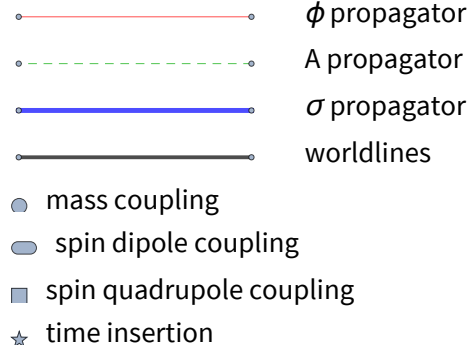 mass coupling
- 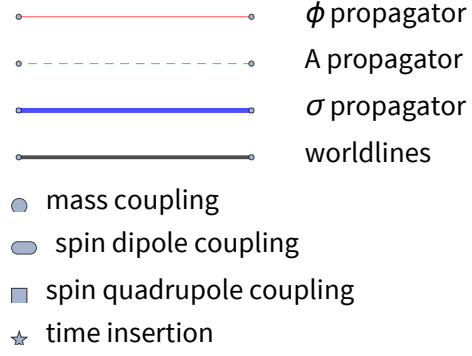 spin dipole coupling
- 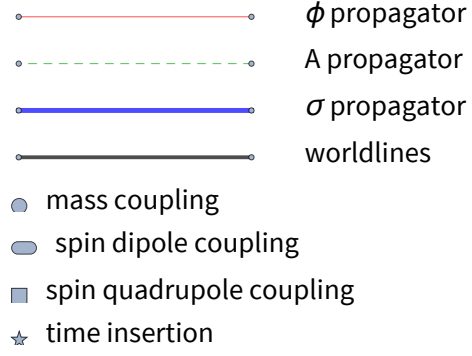 spin quadrupole coupling
- 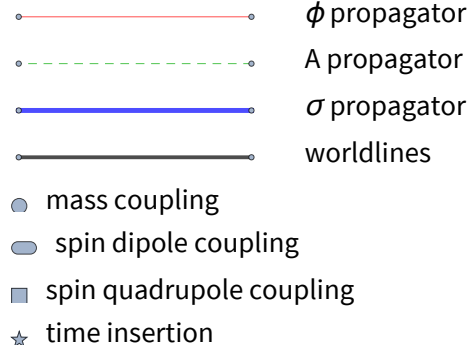 time insertion

$$\begin{aligned}
 & \left\{ \text{DiagS1S1}[2, 1, 1], \right. \\
 & \quad \left. , \frac{2 G^2 m_2 \vec{v}_2 \cdot \vec{v}_2 \left( \hat{n} \times \vec{S}_1 \cdot \vec{v}_2 \right)^2}{r^4} \right\} \\
 & \left\{ \text{DiagS1S1}[2, 1, 2], \right. \\
 & \quad \left. , \frac{G^2 m_2 \left( 4 \vec{v}_2 \cdot \vec{v}_2 \hat{n} \times \vec{S}_1 \cdot \vec{v}_1 \hat{n} \times \vec{S}_1 \cdot \vec{v}_2 - 4 \vec{v}_1 \cdot \vec{v}_2 \left( \hat{n} \times \vec{S}_1 \cdot \vec{v}_2 \right)^2 \right)}{r^4} \right\} \\
 & \left\{ \text{DiagS1S1}[2, 1, 3], \right. \\
 & \quad \left. , \frac{G^2 m_2 \left( 12 \vec{v}_1 \cdot \vec{v}_2 \hat{n} \times \vec{S}_1 \cdot \vec{v}_1 \hat{n} \times \vec{S}_1 \cdot \vec{v}_2 - 12 \vec{v}_2 \cdot \vec{v}_2 \left( \hat{n} \times \vec{S}_1 \cdot \vec{v}_1 \right)^2 \right)}{r^4} \right\}
 \end{aligned}$$

$\{\text{DiagS1S1}[2, 1, 4],$  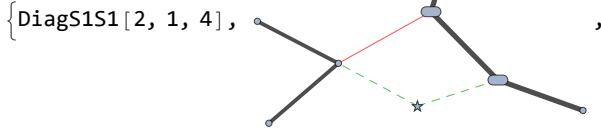 ,

$$G^2 m_2 \left( \frac{1}{r^3} \left( -2 \vec{S}_1 \times \vec{v}_1 \cdot \vec{a}_2 \hat{n} \times \vec{S}_1 \cdot \vec{v}_1 - 2 \vec{S}_1 \times \vec{v}_1 \cdot \vec{v}_2 \hat{n} \times \vec{S}_1 \cdot \vec{a}_1 - 2 \hat{n} \cdot \vec{v}_1 \hat{n} \times \vec{S}_1 \cdot \vec{a}_2 \hat{n} \times \vec{S}_1 \cdot \vec{v}_1 - 2 \hat{n} \cdot \vec{v}_1 \hat{n} \times \vec{S}_1 \cdot \vec{a}_1 \hat{n} \times \vec{S}_1 \cdot \vec{v}_2 - \right. \right. \\ \left. \left. 2 \vec{S}_1 \times \vec{v}_1 \cdot \vec{v}_2 \hat{n} \times \vec{S}_1 \cdot \vec{v}_1 - 2 \vec{S}_1 \times \vec{v}_1 \cdot \vec{v}_2 \hat{n} \times \vec{S}_1 \cdot \vec{v}_2 - 6 \hat{n} \cdot \vec{v}_1 \hat{n} \times \vec{S}_1 \cdot \vec{v}_2 \hat{n} \times \vec{S}_1 \cdot \vec{v}_1 - 2 \hat{n} \cdot \vec{v}_1 \hat{n} \times \vec{S}_1 \cdot \vec{v}_1 \hat{n} \times \vec{S}_1 \cdot \vec{v}_2 + \right. \right. \\ \left. \left. 8 \hat{n} \cdot \vec{v}_2 \hat{n} \times \vec{S}_1 \cdot \vec{v}_2 \hat{n} \times \vec{S}_1 \cdot \vec{v}_1 \right) + \frac{2 \hat{n} \times \vec{S}_1 \cdot \vec{a}_1 \hat{n} \times \vec{S}_1 \cdot \vec{v}_2 + 2 \hat{n} \times \vec{S}_1 \cdot \vec{a}_2 \hat{n} \times \vec{S}_1 \cdot \vec{v}_1 + 2 \hat{n} \times \vec{S}_1 \cdot \vec{v}_1 \hat{n} \times \vec{S}_1 \cdot \vec{v}_2}{r^2} + \frac{1}{r^4} \right. \\ \left. \left( 6 \hat{n} \cdot \vec{v}_1 \vec{S}_1 \times \vec{v}_1 \cdot \vec{v}_2 \hat{n} \times \vec{S}_1 \cdot \vec{v}_1 + 2 \hat{n} \cdot \vec{v}_1 \vec{S}_1 \times \vec{v}_1 \cdot \vec{v}_2 \hat{n} \times \vec{S}_1 \cdot \vec{v}_2 - 8 \hat{n} \cdot \vec{v}_2 \vec{S}_1 \times \vec{v}_1 \cdot \vec{v}_2 \hat{n} \times \vec{S}_1 \cdot \vec{v}_1 + 6 (\hat{n} \cdot \vec{v}_1)^2 \right. \right. \\ \left. \left. \hat{n} \times \vec{S}_1 \cdot \vec{v}_1 \hat{n} \times \vec{S}_1 \cdot \vec{v}_2 - 12 \hat{n} \cdot \vec{v}_1 \hat{n} \cdot \vec{v}_2 \hat{n} \times \vec{S}_1 \cdot \vec{v}_1 \hat{n} \times \vec{S}_1 \cdot \vec{v}_2 + 2 \vec{v}_1 \cdot \vec{v}_2 \hat{n} \times \vec{S}_1 \cdot \vec{v}_1 \hat{n} \times \vec{S}_1 \cdot \vec{v}_2 + 2 (\vec{S}_1 \times \vec{v}_1 \cdot \vec{v}_2)^2 \right) \right\}$$

$\{\text{DiagS1S1}[2, 1, 5],$  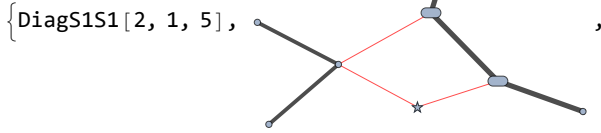 ,

$$G^2 m_2 \left( \frac{1}{r^3} \left( 2 \vec{S}_1 \times \vec{a}_1 \cdot \vec{v}_2 \hat{n} \times \vec{S}_1 \cdot \vec{v}_1 + 2 \vec{S}_1 \times \vec{v}_1 \cdot \vec{v}_2 \hat{n} \times \vec{S}_1 \cdot \vec{a}_1 + 8 \hat{n} \cdot \vec{v}_1 \hat{n} \times \vec{S}_1 \cdot \vec{a}_1 \hat{n} \times \vec{S}_1 \cdot \vec{v}_1 - 8 \hat{n} \cdot \vec{v}_2 \hat{n} \times \vec{S}_1 \cdot \vec{a}_1 \hat{n} \times \vec{S}_1 \cdot \vec{v}_1 + \right. \right. \\ \left. \left. 2 \vec{S}_1 \times \vec{v}_1 \cdot \vec{v}_2 \hat{n} \times \vec{S}_1 \cdot \vec{v}_1 + 2 \vec{S}_1 \times \vec{v}_1 \cdot \vec{v}_2 \hat{n} \times \vec{S}_1 \cdot \vec{v}_1 + 8 \hat{n} \cdot \vec{v}_1 \hat{n} \times \vec{S}_1 \cdot \vec{v}_1 \hat{n} \times \vec{S}_1 \cdot \vec{v}_1 - 8 \hat{n} \cdot \vec{v}_2 \hat{n} \times \vec{S}_1 \cdot \vec{v}_1 \hat{n} \times \vec{S}_1 \cdot \vec{v}_1 \right) + \right. \\ \left. \frac{-4 \hat{n} \times \vec{S}_1 \cdot \vec{a}_1 \hat{n} \times \vec{S}_1 \cdot \vec{v}_1 - 2 (\hat{n} \times \vec{S}_1 \cdot \vec{a}_1)^2 - 2 (\hat{n} \times \vec{S}_1 \cdot \vec{v}_1)^2}{r^2} + \right. \\ \left. \frac{-6 (\hat{n} \cdot \vec{v}_1)^2 (\hat{n} \times \vec{S}_1 \cdot \vec{v}_1)^2 + 12 \hat{n} \cdot \vec{v}_1 \hat{n} \cdot \vec{v}_2 (\hat{n} \times \vec{S}_1 \cdot \vec{v}_1)^2 - 2 \vec{v}_1 \cdot \vec{v}_2 (\hat{n} \times \vec{S}_1 \cdot \vec{v}_1)^2 - 4 \hat{n} \cdot \vec{v}_1 \vec{S}_1 \times \vec{v}_1 \cdot \vec{v}_2 \hat{n} \times \vec{S}_1 \cdot \vec{v}_1}{r^4} \right\}$$

$\{\text{DiagS1S1}[2, 1, 6],$  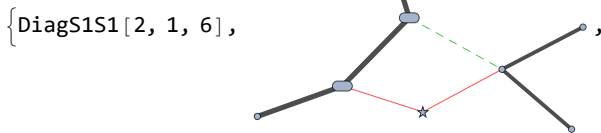 ,

$$G^2 m_2 \left( \frac{1}{r^3} \left( -2 \vec{S}_1 \times \vec{a}_1 \cdot \vec{v}_2 \hat{n} \times \vec{S}_1 \cdot \vec{v}_2 - 2 \vec{S}_1 \times \vec{v}_1 \cdot \vec{v}_2 \hat{n} \times \vec{S}_1 \cdot \vec{a}_1 - 2 \hat{n} \cdot \vec{v}_1 \hat{n} \times \vec{S}_1 \cdot \vec{a}_2 \hat{n} \times \vec{S}_1 \cdot \vec{v}_1 - \right. \right.$$

$$\begin{aligned}
& 6 \hat{n} \cdot \vec{v}_1 \hat{n} \times \vec{S}_1 \cdot \vec{a}_1 \hat{n} \times \vec{S}_1 \cdot \vec{v}_2 + 8 \hat{n} \cdot \vec{v}_2 \hat{n} \times \vec{S}_1 \cdot \vec{a}_1 \hat{n} \times \vec{S}_1 \cdot \vec{v}_2 - 2 \vec{S}_1 \times \vec{v}_1 \cdot \vec{v}_2 \hat{n} \times \vec{S}_1 \cdot \vec{v}_2 - 2 \vec{S}_1 \times \vec{v}_1 \cdot \vec{v}_2 \hat{n} \times \vec{S}_1 \cdot \vec{v}_1 - \\
& 2 \hat{n} \cdot \vec{v}_1 \hat{n} \times \vec{S}_1 \cdot \vec{v}_2 \hat{n} \times \vec{S}_1 \cdot \vec{v}_1 - 6 \hat{n} \cdot \vec{v}_1 \hat{n} \times \vec{S}_1 \cdot \vec{v}_1 \hat{n} \times \vec{S}_1 \cdot \vec{v}_2 + 8 \hat{n} \cdot \vec{v}_2 \hat{n} \times \vec{S}_1 \cdot \vec{v}_1 \hat{n} \times \vec{S}_1 \cdot \vec{v}_2 \Big) + \\
& \frac{2 \hat{n} \times \vec{S}_1 \cdot \vec{a}_1 \hat{n} \times \vec{S}_1 \cdot \vec{v}_2 + 2 \hat{n} \times \vec{S}_1 \cdot \vec{a}_2 \hat{n} \times \vec{S}_1 \cdot \vec{v}_1 + 2 \hat{n} \times \vec{S}_1 \cdot \vec{a}_1 \hat{n} \times \vec{S}_1 \cdot \vec{a}_2 + 2 \hat{n} \times \vec{S}_1 \cdot \vec{v}_1 \hat{n} \times \vec{S}_1 \cdot \vec{v}_2}{r^2} + \frac{1}{r^4} \\
& \left( 6 (\hat{n} \cdot \vec{v}_1)^2 \hat{n} \times \vec{S}_1 \cdot \vec{v}_1 \hat{n} \times \vec{S}_1 \cdot \vec{v}_2 + 2 \hat{n} \cdot \vec{v}_1 \vec{S}_1 \times \vec{v}_1 \cdot \vec{v}_2 \hat{n} \times \vec{S}_1 \cdot \vec{v}_1 + 2 \hat{n} \cdot \vec{v}_1 \vec{S}_1 \times \vec{v}_1 \cdot \vec{v}_2 \hat{n} \times \vec{S}_1 \cdot \vec{v}_2 - \right. \\
& \left. 12 \hat{n} \cdot \vec{v}_2 \hat{n} \cdot \vec{v}_1 \hat{n} \times \vec{S}_1 \cdot \vec{v}_1 \hat{n} \times \vec{S}_1 \cdot \vec{v}_2 + 2 \vec{v}_1 \cdot \vec{v}_2 \hat{n} \times \vec{S}_1 \cdot \vec{v}_1 \hat{n} \times \vec{S}_1 \cdot \vec{v}_2 \right) \Big\}
\end{aligned}$$

{DiagS1S1[2, 1, 7],

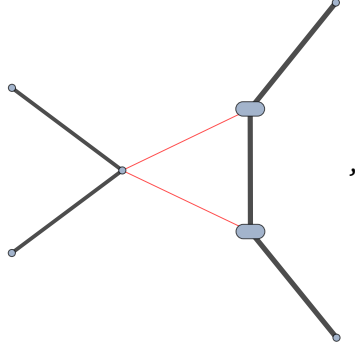

$$G^2 m_2 \left\{ \frac{9 \vec{v}_2 \cdot \vec{v}_2 (\hat{n} \times \vec{S}_1 \cdot \vec{v}_1)^2 - 2 \vec{v}_1 \cdot \vec{v}_1 (\hat{n} \times \vec{S}_1 \cdot \vec{v}_1)^2}{r^4} - \frac{4 \vec{S}_1 \times \vec{v}_1 \cdot \vec{a}_1 \hat{n} \times \vec{S}_1 \cdot \vec{v}_1}{r^3} \right\}$$

{DiagS1S1[2, 1, 8],

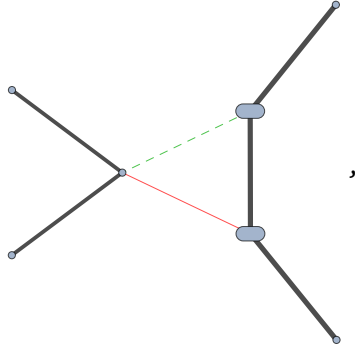

$$\begin{aligned}
& G^2 m_2 \left\{ \frac{-8 \vec{S}_1 \times \vec{a}_1 \cdot \vec{v}_2 \hat{n} \times \vec{S}_1 \cdot \vec{v}_1 + 4 \vec{S}_1 \times \vec{v}_1 \cdot \vec{a}_1 \hat{n} \times \vec{S}_1 \cdot \vec{v}_2 - 8 \vec{S}_1 \times \vec{v}_1 \cdot \vec{v}_2 \hat{n} \times \vec{S}_1 \cdot \vec{v}_1}{r^3} + \right. \\
& \left. \frac{6 \vec{v}_1 \cdot \vec{v}_2 (\hat{n} \times \vec{S}_1 \cdot \vec{v}_1)^2 + 2 \hat{n} \cdot \vec{v}_1 \vec{S}_1 \times \vec{v}_1 \cdot \vec{v}_2 \hat{n} \times \vec{S}_1 \cdot \vec{v}_1 + 2 \vec{v}_1 \cdot \vec{v}_1 \hat{n} \times \vec{S}_1 \cdot \vec{v}_2 \hat{n} \times \vec{S}_1 \cdot \vec{v}_1 - 6 \vec{v}_2 \cdot \vec{v}_2 \hat{n} \times \vec{S}_1 \cdot \vec{v}_2 \hat{n} \times \vec{S}_1 \cdot \vec{v}_1}{r^4} \right\}
\end{aligned}$$

{DiagS1S1[2, 2, 1],

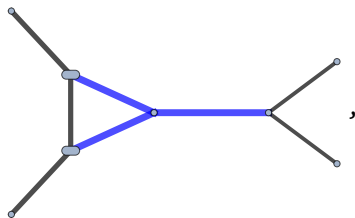

,  $\frac{1}{r^4}$

$$G^2 m_2 \left( -\frac{9}{4} (\hat{n} \cdot \vec{v}_2)^2 (\hat{n} \times \vec{S}_1 \cdot \vec{v}_1)^2 + \frac{27}{4} \vec{v}_2 \cdot \vec{v}_2 (\hat{n} \times \vec{S}_1 \cdot \vec{v}_1)^2 + 3 \hat{n} \cdot \vec{v}_2 \vec{S}_1 \times \vec{v}_1 \cdot \vec{v}_2 \hat{n} \times \vec{S}_1 \cdot \vec{v}_1 - \right.$$

$$\begin{aligned} & 8 \vec{v}_1 \cdot \vec{v}_2 \hat{n} \times \vec{S}_1 \cdot \vec{v}_2 \hat{n} \times \vec{S}_1 \cdot \vec{v}_1 - 2 \hat{n} \cdot \vec{v}_1 \vec{S}_1 \times \vec{v}_1 \cdot \vec{v}_2 \hat{n} \times \vec{S}_1 \cdot \vec{v}_2 + 3 \vec{v}_1 \cdot \vec{v}_1 \left( \hat{n} \times \vec{S}_1 \cdot \vec{v}_2 \right)^2 - \frac{3}{4} \left( \hat{n} \cdot \vec{v}_2 \right)^2 \left( \vec{S}_1 \cdot \vec{v}_1 \right)^2 + \\ & \left( \vec{v}_1 \cdot \vec{v}_2 \right)^2 \left( \hat{n} \cdot \vec{S}_1 \right)^2 - \frac{9}{4} \vec{v}_1 \cdot \vec{v}_1 \left( \hat{n} \cdot \vec{S}_1 \right)^2 \left( \hat{n} \cdot \vec{v}_2 \right)^2 + \frac{5}{2} \vec{S}_1 \cdot \vec{S}_1 \vec{v}_1 \cdot \vec{v}_1 \left( \hat{n} \cdot \vec{v}_2 \right)^2 - \vec{v}_1 \cdot \vec{v}_1 \hat{n} \cdot \vec{S}_1 \hat{n} \cdot \vec{v}_2 \vec{S}_1 \cdot \vec{v}_2 + \\ & 6 \vec{S}_1 \cdot \vec{S}_1 \vec{v}_1 \cdot \vec{v}_2 \hat{n} \cdot \vec{v}_1 \hat{n} \cdot \vec{v}_2 - 2 \vec{v}_1 \cdot \vec{v}_2 \hat{n} \cdot \vec{S}_1 \hat{n} \cdot \vec{v}_2 \vec{S}_1 \cdot \vec{v}_1 - 4 \vec{v}_1 \cdot \vec{v}_2 \hat{n} \cdot \vec{S}_1 \hat{n} \cdot \vec{v}_1 \vec{S}_1 \cdot \vec{v}_2 - \\ & 6 \vec{S}_1 \cdot \vec{S}_1 \vec{v}_2 \cdot \vec{v}_2 \left( \hat{n} \cdot \vec{v}_1 \right)^2 + 6 \vec{v}_2 \cdot \vec{v}_2 \hat{n} \cdot \vec{S}_1 \hat{n} \cdot \vec{v}_1 \vec{S}_1 \cdot \vec{v}_1 + \frac{3}{4} \vec{v}_1 \cdot \vec{v}_1 \vec{v}_2 \cdot \vec{v}_2 \left( \hat{n} \cdot \vec{S}_1 \right)^2 - \left( \vec{S}_1 \times \vec{v}_1 \cdot \vec{v}_2 \right)^2 - \\ & \vec{S}_1 \cdot \vec{S}_1 \left( \vec{v}_1 \cdot \vec{v}_2 \right)^2 + \vec{v}_1 \cdot \vec{v}_1 \left( \vec{S}_1 \cdot \vec{v}_2 \right)^2 + \vec{v}_1 \cdot \vec{v}_2 \vec{S}_1 \cdot \vec{v}_1 \vec{S}_1 \cdot \vec{v}_2 - \frac{3}{4} \vec{v}_2 \cdot \vec{v}_2 \left( \vec{S}_1 \cdot \vec{v}_1 \right)^2 - \frac{1}{2} \vec{S}_1 \cdot \vec{S}_1 \vec{v}_1 \cdot \vec{v}_1 \vec{v}_2 \cdot \vec{v}_2 \Big\} \end{aligned}$$

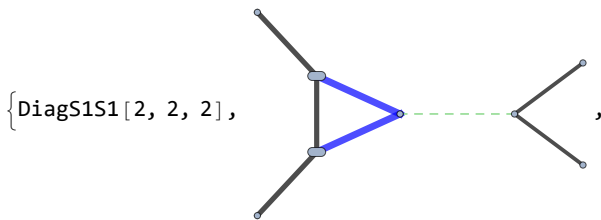

[illegible]

{DiagS1S1[2, 2, 3],

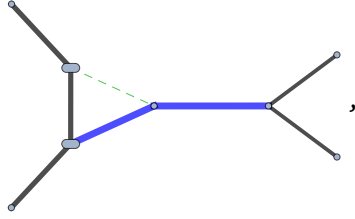

$$\begin{aligned}
 & G^2 \left( \frac{1}{r^3} \left( 2 \hat{n} \cdot \vec{a}_1 \left( \hat{n} \times \vec{S}_1 \cdot \vec{v}_2 \right)^2 - 4 \vec{S}_1 \times \vec{v}_1 \cdot \vec{v}_2 \hat{n} \times \vec{S}_1 \cdot \vec{v}_2 - 2 \vec{S}_1 \times \vec{a}_1 \cdot \vec{v}_2 \hat{n} \times \vec{S}_1 \cdot \vec{v}_2 - \vec{S}_1 \times \vec{v}_1 \cdot \vec{a}_2 \hat{n} \times \vec{S}_1 \cdot \vec{v}_2 + \right. \right. \\
 & 4 \hat{n} \times \vec{S}_1 \cdot \vec{v}_1 \hat{n} \cdot \vec{a}_2 \hat{n} \times \vec{S}_1 \cdot \vec{v}_2 + 10 \hat{n} \times \vec{S}_1 \cdot \vec{v}_1 \hat{n} \cdot \vec{v}_2 \hat{n} \times \vec{S}_1 \cdot \vec{v}_2 + 6 \hat{n} \times \vec{S}_1 \cdot \vec{a}_1 \hat{n} \cdot \vec{v}_2 \hat{n} \times \vec{S}_1 \cdot \vec{v}_2 + \hat{n} \cdot \vec{a}_1 \left( \vec{S}_1 \cdot \vec{v}_2 \right)^2 - \\
 & \hat{n} \times \vec{S}_1 \cdot \vec{v}_2 \vec{S}_1 \times \vec{v}_1 \cdot \vec{v}_2 - \hat{n} \times \vec{S}_1 \cdot \vec{a}_2 \vec{S}_1 \times \vec{v}_1 \cdot \vec{v}_2 - 2 \hat{n} \times \vec{S}_1 \cdot \vec{v}_2 \hat{n} \times \vec{S}_1 \cdot \vec{v}_1 \hat{n} \cdot \vec{v}_2 + 4 \hat{n} \times \vec{S}_1 \cdot \vec{a}_2 \hat{n} \times \vec{S}_1 \cdot \vec{v}_1 \hat{n} \cdot \vec{v}_2 + \\
 & 6 \left( \hat{n} \cdot \vec{S}_1 \right)^2 \hat{n} \cdot \vec{v}_2 \vec{a}_1 \cdot \vec{v}_2 + \hat{n} \cdot \vec{v}_2 \vec{a}_1 \cdot \vec{v}_2 \vec{S}_1 \cdot \vec{S}_1 + 5 \hat{n} \cdot \vec{v}_2 \vec{S}_1 \cdot \vec{v}_2 \vec{S}_1 \cdot \vec{v}_1 + 2 \hat{n} \cdot \vec{v}_2 \vec{S}_1 \cdot \vec{a}_2 \vec{S}_1 \cdot \vec{v}_1 - \\
 & \hat{n} \cdot \vec{v}_2 \vec{S}_1 \cdot \vec{v}_1 \vec{S}_1 \cdot \vec{v}_2 - 4 \hat{n} \cdot \vec{S}_1 \vec{a}_1 \cdot \vec{v}_2 \vec{S}_1 \cdot \vec{v}_2 + 3 \hat{n} \cdot \vec{v}_2 \vec{S}_1 \cdot \vec{a}_1 \vec{S}_1 \cdot \vec{v}_2 + 2 \hat{n} \cdot \vec{a}_2 \vec{S}_1 \cdot \vec{v}_1 \vec{S}_1 \cdot \vec{v}_2 + \\
 & 4 \left( \hat{n} \cdot \vec{S}_1 \right)^2 \hat{n} \cdot \vec{v}_2 \vec{v}_1 \cdot \vec{a}_2 - 2 \hat{n} \cdot \vec{S}_1 \vec{S}_1 \cdot \vec{v}_2 \vec{v}_1 \cdot \vec{a}_2 + 4 \hat{n} \cdot \vec{a}_2 \left( \hat{n} \cdot \vec{S}_1 \right)^2 \vec{v}_1 \cdot \vec{v}_2 + 8 \hat{n} \cdot \vec{S}_1 \hat{n} \cdot \vec{S}_1 \hat{n} \cdot \vec{v}_2 \vec{v}_1 \cdot \vec{v}_2 - \\
 & 2 \hat{n} \cdot \vec{S}_1 \vec{S}_1 \cdot \vec{v}_2 \vec{v}_1 \cdot \vec{v}_2 + 2 \hat{n} \cdot \vec{v}_2 \vec{S}_1 \cdot \vec{S}_1 \vec{v}_1 \cdot \vec{v}_2 - 2 \hat{n} \cdot \vec{S}_1 \vec{S}_1 \cdot \vec{a}_2 \vec{v}_1 \cdot \vec{v}_2 - 4 \hat{n} \cdot \vec{S}_1 \vec{S}_1 \cdot \vec{v}_2 \vec{v}_1 \cdot \vec{v}_2 + \\
 & 2 \hat{n} \cdot \vec{a}_1 \left( \hat{n} \cdot \vec{S}_1 \right)^2 \vec{v}_2 \cdot \vec{v}_2 - 2 \hat{n} \cdot \vec{v}_1 \vec{S}_1 \cdot \vec{S}_1 \vec{v}_2 \cdot \vec{v}_2 - \hat{n} \cdot \vec{a}_1 \vec{S}_1 \cdot \vec{S}_1 \vec{v}_2 \cdot \vec{v}_2 + 2 \hat{n} \cdot \vec{S}_1 \vec{S}_1 \cdot \vec{v}_1 \vec{v}_2 \cdot \vec{v}_2 \Big) + \\
 & \frac{1}{r^4} \left( -4 \vec{v}_2 \cdot \vec{v}_2 \left( \hat{n} \times \vec{S}_1 \cdot \vec{v}_1 \right)^2 + 24 \hat{n} \times \vec{S}_1 \cdot \vec{v}_2 \left( \hat{n} \cdot \vec{v}_2 \right)^2 \hat{n} \times \vec{S}_1 \cdot \vec{v}_1 - 10 \vec{S}_1 \times \vec{v}_1 \cdot \vec{v}_2 \hat{n} \cdot \vec{v}_2 \hat{n} \times \vec{S}_1 \cdot \vec{v}_1 - \right. \\
 & 24 \hat{n} \times \vec{S}_1 \cdot \vec{v}_2 \hat{n} \cdot \vec{v}_1 \hat{n} \cdot \vec{v}_2 \hat{n} \times \vec{S}_1 \cdot \vec{v}_1 + 8 \hat{n} \times \vec{S}_1 \cdot \vec{v}_2 \vec{v}_1 \cdot \vec{v}_2 \hat{n} \times \vec{S}_1 \cdot \vec{v}_1 - 4 \hat{n} \times \vec{S}_1 \cdot \vec{v}_2 \vec{v}_2 \cdot \vec{v}_2 \hat{n} \times \vec{S}_1 \cdot \vec{v}_1 + \\
 & 4 \left( \vec{S}_1 \times \vec{v}_1 \cdot \vec{v}_2 \right)^2 + 4 \left( \hat{n} \cdot \vec{S}_1 \right)^2 \left( \vec{v}_1 \cdot \vec{v}_2 \right)^2 + 10 \hat{n} \times \vec{S}_1 \cdot \vec{v}_2 \vec{S}_1 \times \vec{v}_1 \cdot \vec{v}_2 \hat{n} \cdot \vec{v}_1 - 8 \hat{n} \times \vec{S}_1 \cdot \vec{v}_2 \vec{S}_1 \times \vec{v}_1 \cdot \vec{v}_2 \hat{n} \cdot \vec{v}_2 + \\
 & 8 \left( \hat{n} \cdot \vec{v}_2 \right)^2 \vec{S}_1 \cdot \vec{v}_1 \vec{S}_1 \cdot \vec{v}_2 - 8 \hat{n} \cdot \vec{v}_1 \hat{n} \cdot \vec{v}_2 \vec{S}_1 \cdot \vec{v}_1 \vec{S}_1 \cdot \vec{v}_2 + 24 \left( \hat{n} \cdot \vec{S}_1 \right)^2 \left( \hat{n} \cdot \vec{v}_2 \right)^2 \vec{v}_1 \cdot \vec{v}_2 + 2 \left( \vec{S}_1 \cdot \vec{v}_2 \right)^2 \vec{v}_1 \cdot \vec{v}_2 - \\
 & 24 \left( \hat{n} \cdot \vec{S}_1 \right)^2 \hat{n} \cdot \vec{v}_1 \hat{n} \cdot \vec{v}_2 \vec{v}_1 \cdot \vec{v}_2 - 4 \hat{n} \cdot \vec{v}_1 \hat{n} \cdot \vec{v}_2 \vec{S}_1 \cdot \vec{S}_1 \vec{v}_1 \cdot \vec{v}_2 + 8 \hat{n} \cdot \vec{S}_1 \hat{n} \cdot \vec{v}_2 \vec{S}_1 \cdot \vec{v}_1 \vec{v}_1 \cdot \vec{v}_2 + \\
 & 12 \hat{n} \cdot \vec{S}_1 \hat{n} \cdot \vec{v}_1 \vec{S}_1 \cdot \vec{v}_2 \vec{v}_1 \cdot \vec{v}_2 - 16 \hat{n} \cdot \vec{S}_1 \hat{n} \cdot \vec{v}_2 \vec{S}_1 \cdot \vec{v}_2 \vec{v}_1 \cdot \vec{v}_2 + 4 \left( \hat{n} \cdot \vec{v}_1 \right)^2 \vec{S}_1 \cdot \vec{S}_1 \vec{v}_2 \cdot \vec{v}_2 - \\
 & \left. 4 \hat{n} \cdot \vec{S}_1 \hat{n} \cdot \vec{v}_1 \vec{S}_1 \cdot \vec{v}_1 \vec{v}_2 \cdot \vec{v}_2 - 2 \vec{S}_1 \cdot \vec{v}_1 \vec{S}_1 \cdot \vec{v}_2 \vec{v}_2 \cdot \vec{v}_2 - 4 \left( \hat{n} \cdot \vec{S}_1 \right)^2 \vec{v}_1 \cdot \vec{v}_2 \vec{v}_2 \cdot \vec{v}_2 \right) \Big) m_2 \Big\}
 \end{aligned}$$

{DiagS1S1[2, 2, 4],

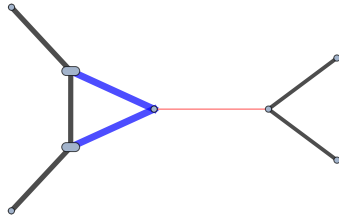

,  $G^2 m_2$

$$\begin{aligned}
 & \left( \frac{1}{r^3} \left( 2 \vec{S}_1 \times \vec{v}_1 \cdot \vec{a}_1 \hat{n} \times \vec{S}_1 \cdot \vec{v}_1 + 2 \hat{n} \cdot \vec{v}_1 \hat{n} \times \vec{S}_1 \cdot \vec{a}_1 \hat{n} \times \vec{S}_1 \cdot \vec{v}_1 + 2 \vec{v}_1 \cdot \vec{a}_1 \left( \hat{n} \cdot \vec{S}_1 \right)^2 \hat{n} \cdot \vec{v}_1 - \vec{v}_1 \cdot \vec{a}_1 \hat{n} \cdot \vec{S}_1 \vec{S}_1 \cdot \vec{v}_1 + \vec{S}_1 \cdot \vec{a}_1 \hat{n} \cdot \vec{v}_1 \right. \right. \\
 & \left. \vec{S}_1 \cdot \vec{v}_1 + 2 \hat{n} \cdot \vec{v}_1 \hat{n} \times \vec{S}_1 \cdot \vec{v}_1 \hat{n} \times \vec{S}_1 \cdot \vec{v}_1 + 2 \vec{v}_1 \cdot \vec{v}_1 \hat{n} \cdot \vec{S}_1 \hat{n} \cdot \vec{S}_1 \hat{n} \cdot \vec{v}_1 + \hat{n} \cdot \vec{v}_1 \vec{S}_1 \cdot \vec{v}_1 \vec{S}_1 \cdot \vec{v}_1 - \vec{v}_1 \cdot \vec{v}_1 \hat{n} \cdot \vec{S}_1 \vec{S}_1 \cdot \vec{v}_1 \right) + \frac{1}{r^2} \\
 & \left( -2 \hat{n} \times \vec{S}_1 \cdot \vec{a}_1 \hat{n} \times \vec{S}_1 \cdot \vec{v}_1 + \hat{n} \times \vec{S}_1 \cdot \vec{a}_1 \hat{n} \times \vec{S}_1 \cdot \vec{v}_1 - \vec{v}_1 \cdot \vec{a}_1 \hat{n} \cdot \vec{S}_1 \hat{n} \cdot \vec{S}_1 - \frac{1}{2} \left( \hat{n} \times \vec{S}_1 \cdot \vec{a}_1 \right)^2 - \frac{1}{2} \vec{a}_1 \cdot \vec{a}_1 \left( \hat{n} \cdot \vec{S}_1 \right)^2 + \right. \\
 & \left. \vec{S}_1 \cdot \vec{a}_1 \vec{S}_1 \cdot \vec{v}_1 - 2 \vec{S}_1 \cdot \vec{a}_1 \vec{S}_1 \cdot \vec{v}_1 - \frac{1}{2} \left( \vec{S}_1 \cdot \vec{a}_1 \right)^2 - \frac{1}{2} \left( \hat{n} \times \vec{S}_1 \cdot \vec{v}_1 \right)^2 - \frac{1}{2} \vec{v}_1 \cdot \vec{v}_1 \left( \hat{n} \cdot \vec{S}_1 \right)^2 - \frac{1}{2} \left( \vec{S}_1 \cdot \vec{v}_1 \right)^2 \right) + \\
 & \frac{1}{r^4} \left( -\frac{9}{4} \left( \hat{n} \cdot \vec{v}_1 \right)^2 \left( \hat{n} \times \vec{S}_1 \cdot \vec{v}_1 \right)^2 + \frac{3}{4} \vec{v}_1 \cdot \vec{v}_1 \left( \hat{n} \times \vec{S}_1 \cdot \vec{v}_1 \right)^2 - \frac{3}{4} \left( \hat{n} \cdot \vec{v}_1 \right)^2 \left( \vec{S}_1 \cdot \vec{v}_1 \right)^2 + \right. \\
 & \left. \frac{3}{4} \left( \vec{v}_1 \cdot \vec{v}_1 \right)^2 \left( \hat{n} \cdot \vec{S}_1 \right)^2 - \frac{9}{4} \vec{v}_1 \cdot \vec{v}_1 \left( \hat{n} \cdot \vec{S}_1 \right)^2 \left( \hat{n} \cdot \vec{v}_1 \right)^2 + \frac{1}{2} \vec{S}_1 \cdot \vec{S}_1 \vec{v}_1 \cdot \vec{v}_1 \left( \hat{n} \cdot \vec{v}_1 \right)^2 + \right.
 \end{aligned}$$

$$\vec{v}_1 \cdot \vec{v}_1 \hat{n} \cdot \vec{S}_1 \hat{n} \cdot \vec{v}_1 \vec{S}_1 \cdot \vec{v}_1 - \frac{1}{2} \vec{S}_1 \cdot \vec{S}_1 (\vec{v}_1 \cdot \vec{v}_1)^2 + \frac{1}{4} \vec{v}_1 \cdot \vec{v}_1 (\vec{S}_1 \cdot \vec{v}_1)^2 \Big) \Big) \Big\}$$

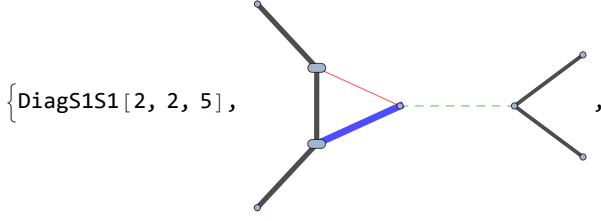

$$G^2 \left( \frac{1}{r^3} \left( 4 \hat{n} \times \vec{S}_1 \cdot \vec{v}_2 \vec{S}_1 \times \vec{v}_1 \cdot \vec{a}_1 + 4 \hat{n} \times \vec{S}_1 \cdot \vec{v}_1 \vec{S}_1 \times \vec{v}_1 \cdot \vec{a}_2 + 4 \hat{n} \times \vec{S}_1 \cdot \vec{v}_1 \vec{S}_1 \times \vec{v}_1 \cdot \vec{v}_2 + 4 \hat{n} \times \vec{S}_1 \cdot \vec{a}_1 \vec{S}_1 \times \vec{v}_1 \cdot \vec{v}_2 + \right. \right. \\ \left. \left. 8 \hat{n} \times \vec{S}_1 \cdot \vec{a}_2 \hat{n} \times \vec{S}_1 \cdot \vec{v}_1 \hat{n} \cdot \vec{v}_1 + 16 \hat{n} \times \vec{S}_1 \cdot \vec{v}_1 \hat{n} \times \vec{S}_1 \cdot \vec{v}_2 \hat{n} \cdot \vec{v}_1 + 16 \hat{n} \times \vec{S}_1 \cdot \vec{a}_1 \hat{n} \times \vec{S}_1 \cdot \vec{v}_2 \hat{n} \cdot \vec{v}_1 - 8 \hat{n} \cdot \vec{v}_1 \vec{a}_1 \cdot \vec{v}_2 \vec{S}_1 \cdot \vec{S}_1 + \right. \right. \\ \left. \left. 8 \hat{n} \cdot \vec{v}_1 \vec{S}_1 \cdot \vec{v}_2 \vec{S}_1 \cdot \vec{v}_1 + 4 \hat{n} \cdot \vec{v}_1 \vec{S}_1 \cdot \vec{a}_2 \vec{S}_1 \cdot \vec{v}_1 + 8 \hat{n} \cdot \vec{v}_1 \vec{S}_1 \cdot \vec{a}_1 \vec{S}_1 \cdot \vec{v}_2 - 8 \hat{n} \cdot \vec{v}_1 \vec{S}_1 \cdot \vec{S}_1 \vec{v}_1 \cdot \vec{a}_2 + 4 \hat{n} \cdot \vec{S}_1 \vec{S}_1 \cdot \vec{v}_1 \right. \right. \\ \left. \left. \vec{v}_1 \cdot \vec{a}_2 - 12 \hat{n} \cdot \vec{v}_1 \vec{S}_1 \cdot \vec{S}_1 \vec{v}_1 \cdot \vec{v}_2 + 4 \hat{n} \cdot \vec{S}_1 \vec{S}_1 \cdot \vec{a}_1 \vec{v}_1 \cdot \vec{v}_2 - 4 \hat{n} \cdot \vec{a}_1 \vec{S}_1 \cdot \vec{S}_1 \vec{v}_1 \cdot \vec{v}_2 + 4 \hat{n} \cdot \vec{S}_1 \vec{S}_1 \cdot \vec{v}_1 \vec{v}_1 \cdot \vec{v}_2 \right) + \right. \\ \left. \frac{1}{r^4} \left( -8 \vec{v}_1 \cdot \vec{v}_2 (\hat{n} \times \vec{S}_1 \cdot \vec{v}_1)^2 - 48 \hat{n} \times \vec{S}_1 \cdot \vec{v}_2 (\hat{n} \cdot \vec{v}_1)^2 \hat{n} \times \vec{S}_1 \cdot \vec{v}_1 - 24 \vec{S}_1 \times \vec{v}_1 \cdot \vec{v}_2 \hat{n} \cdot \vec{v}_1 \hat{n} \times \vec{S}_1 \cdot \vec{v}_1 + \right. \right. \\ \left. \left. 16 \vec{S}_1 \times \vec{v}_1 \cdot \vec{v}_2 \hat{n} \cdot \vec{v}_2 \hat{n} \times \vec{S}_1 \cdot \vec{v}_1 + 48 \hat{n} \times \vec{S}_1 \cdot \vec{v}_2 \hat{n} \cdot \vec{v}_1 \hat{n} \cdot \vec{v}_2 \hat{n} \times \vec{S}_1 \cdot \vec{v}_1 + 8 \hat{n} \times \vec{S}_1 \cdot \vec{v}_2 \vec{v}_1 \cdot \vec{v}_1 \hat{n} \times \vec{S}_1 \cdot \vec{v}_1 - \right. \right. \\ \left. \left. 8 \hat{n} \times \vec{S}_1 \cdot \vec{v}_2 \vec{v}_1 \cdot \vec{v}_2 \hat{n} \times \vec{S}_1 \cdot \vec{v}_1 - 4 (\vec{S}_1 \times \vec{v}_1 \cdot \vec{v}_2)^2 + 8 \vec{S}_1 \cdot \vec{S}_1 (\vec{v}_1 \cdot \vec{v}_2)^2 - 8 \hat{n} \times \vec{S}_1 \cdot \vec{v}_2 \vec{S}_1 \times \vec{v}_1 \cdot \vec{v}_2 \hat{n} \cdot \vec{v}_1 - \right. \right. \\ \left. \left. 16 (\hat{n} \cdot \vec{v}_1)^2 \vec{S}_1 \cdot \vec{v}_1 \vec{S}_1 \cdot \vec{v}_2 + 16 \hat{n} \cdot \vec{v}_1 \hat{n} \cdot \vec{v}_2 \vec{S}_1 \cdot \vec{v}_1 \vec{S}_1 \cdot \vec{v}_2 + 4 \vec{S}_1 \cdot \vec{v}_1 \vec{S}_1 \cdot \vec{v}_2 \vec{v}_1 \cdot \vec{v}_1 + \right. \right. \\ \left. \left. 24 (\hat{n} \cdot \vec{v}_1)^2 \vec{S}_1 \cdot \vec{S}_1 \vec{v}_1 \cdot \vec{v}_2 - 32 \hat{n} \cdot \vec{v}_1 \hat{n} \cdot \vec{v}_2 \vec{S}_1 \cdot \vec{S}_1 \vec{v}_1 \cdot \vec{v}_2 - 8 \hat{n} \cdot \vec{S}_1 \hat{n} \cdot \vec{v}_1 \vec{S}_1 \cdot \vec{v}_1 \vec{v}_1 \cdot \vec{v}_2 + \right. \right. \\ \left. \left. 16 \hat{n} \cdot \vec{S}_1 \hat{n} \cdot \vec{v}_2 \vec{S}_1 \cdot \vec{v}_1 \vec{v}_1 \cdot \vec{v}_2 - 8 \vec{S}_1 \cdot \vec{v}_1 \vec{S}_1 \cdot \vec{v}_2 \vec{v}_1 \cdot \vec{v}_2 - 4 \vec{S}_1 \cdot \vec{S}_1 \vec{v}_1 \cdot \vec{v}_1 \vec{v}_1 \cdot \vec{v}_2 \right) \right) m_2 \Big\}$$

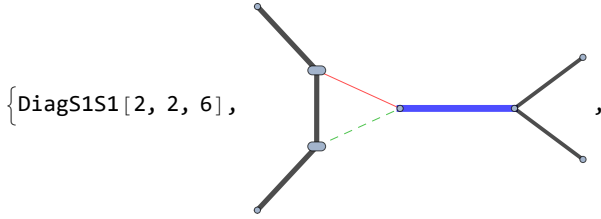

$$G^2 m_2 \left( \frac{1}{r^3} \left( 4 \vec{S}_1 \times \vec{a}_1 \cdot \vec{v}_2 \hat{n} \times \vec{S}_1 \cdot \vec{v}_2 - 8 \hat{n} \cdot \vec{v}_2 \hat{n} \times \vec{S}_1 \cdot \vec{a}_1 \hat{n} \times \vec{S}_1 \cdot \vec{v}_2 + 4 \vec{S}_1 \cdot \vec{S}_1 \vec{a}_1 \cdot \vec{v}_2 \hat{n} \cdot \vec{v}_2 - 4 \vec{S}_1 \cdot \vec{a}_1 \hat{n} \cdot \vec{v}_2 \vec{S}_1 \cdot \vec{v}_2 + \right. \right. \\ \left. \left. 4 \vec{S}_1 \times \vec{v}_1 \cdot \vec{v}_2 \hat{n} \times \vec{S}_1 \cdot \vec{v}_2 + 8 \hat{n} \cdot \vec{v}_2 \hat{n} \times \vec{S}_1 \cdot \vec{v}_2 \hat{n} \times \vec{S}_1 \cdot \vec{v}_1 - 8 \hat{n} \cdot \vec{v}_2 \hat{n} \times \vec{S}_1 \cdot \vec{v}_1 \hat{n} \times \vec{S}_1 \cdot \vec{v}_2 - 4 \hat{n} \cdot \vec{v}_2 \vec{S}_1 \cdot \vec{v}_2 \vec{S}_1 \cdot \vec{v}_1 + \right. \right. \\ \left. \left. 4 \hat{n} \cdot \vec{v}_2 \vec{S}_1 \cdot \vec{v}_1 \vec{S}_1 \cdot \vec{v}_2 \right) + \frac{-8 \hat{n} \cdot \vec{v}_1 \vec{S}_1 \times \vec{v}_1 \cdot \vec{v}_2 \hat{n} \times \vec{S}_1 \cdot \vec{v}_2 + 8 \hat{n} \cdot \vec{v}_2 \vec{S}_1 \times \vec{v}_1 \cdot \vec{v}_2 \hat{n} \times \vec{S}_1 \cdot \vec{v}_1 - 4 (\vec{S}_1 \times \vec{v}_1 \cdot \vec{v}_2)^2}{r^4} \right) \Big\}$$

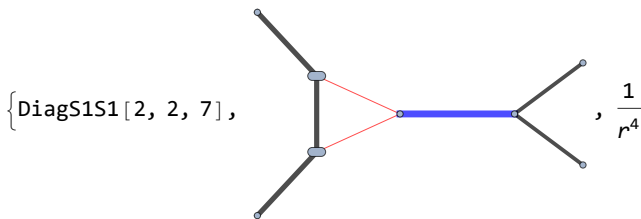

$$G^2 m_2 \left( 9 (\hat{n} \cdot \vec{v}_2)^2 (\hat{n} \times \vec{S}_1 \cdot \vec{v}_1)^2 - 3 \vec{v}_2 \cdot \vec{v}_2 (\hat{n} \times \vec{S}_1 \cdot \vec{v}_1)^2 - 4 \hat{n} \cdot \vec{v}_2 \vec{S}_1 \times \vec{v}_1 \cdot \vec{v}_2 \hat{n} \times \vec{S}_1 \cdot \vec{v}_1 + \right. \\ \left. 3 (\hat{n} \cdot \vec{v}_2)^2 (\vec{S}_1 \cdot \vec{v}_1)^2 - 3 \vec{S}_1 \cdot \vec{S}_1 \vec{v}_1 \cdot \vec{v}_1 (\hat{n} \cdot \vec{v}_2)^2 - \vec{v}_2 \cdot \vec{v}_2 (\vec{S}_1 \cdot \vec{v}_1)^2 + \vec{S}_1 \cdot \vec{S}_1 \vec{v}_1 \cdot \vec{v}_1 \vec{v}_2 \cdot \vec{v}_2 \right) \Big\}$$

$$\{\text{DiagS1S1}[2, 2, 8],$$

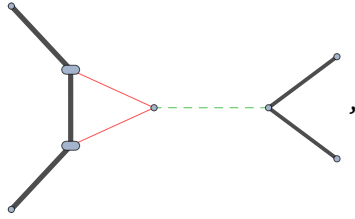

$$G^2 m_2 \left( \frac{1}{r^3} \left( -4 \vec{S}_1 \times \vec{a}_1 \cdot \vec{v}_2 \hat{n} \times \vec{S}_1 \cdot \vec{v}_1 + 8 \hat{n} \cdot \vec{v}_2 \hat{n} \times \vec{S}_1 \cdot \vec{a}_1 \hat{n} \times \vec{S}_1 \cdot \vec{v}_1 + 4 \vec{S}_1 \cdot \vec{a}_1 \hat{n} \cdot \vec{v}_2 \vec{S}_1 \cdot \vec{v}_1 - 4 \vec{S}_1 \cdot \vec{S}_1 \vec{v}_1 \cdot \vec{a}_1 \hat{n} \cdot \vec{v}_2 - \right. \right. \\ \left. \left. 4 \vec{S}_1 \times \vec{v}_1 \cdot \vec{v}_2 \hat{n} \times \vec{S}_1 \cdot \vec{v}_1 + 8 \hat{n} \cdot \vec{v}_2 \hat{n} \times \vec{S}_1 \cdot \vec{v}_1 \hat{n} \times \vec{S}_1 \cdot \vec{v}_1 + 4 \hat{n} \cdot \vec{v}_2 \vec{S}_1 \cdot \vec{v}_1 \vec{S}_1 \cdot \vec{v}_1 - 4 \vec{S}_1 \cdot \vec{S}_1 \vec{v}_1 \cdot \vec{v}_1 \hat{n} \cdot \vec{v}_2 \right) + \right. \\ \left. \frac{1}{r^4} \left( -18 \hat{n} \cdot \vec{v}_1 \hat{n} \cdot \vec{v}_2 \left( \hat{n} \times \vec{S}_1 \cdot \vec{v}_1 \right)^2 + 6 \vec{v}_1 \cdot \vec{v}_2 \left( \hat{n} \times \vec{S}_1 \cdot \vec{v}_1 \right)^2 + 4 \hat{n} \cdot \vec{v}_1 \vec{S}_1 \times \vec{v}_1 \cdot \vec{v}_2 \hat{n} \times \vec{S}_1 \cdot \vec{v}_1 - \right. \right. \\ \left. \left. 6 \hat{n} \cdot \vec{v}_1 \hat{n} \cdot \vec{v}_2 \left( \vec{S}_1 \cdot \vec{v}_1 \right)^2 + 6 \vec{S}_1 \cdot \vec{S}_1 \vec{v}_1 \cdot \vec{v}_1 \hat{n} \cdot \vec{v}_1 \hat{n} \cdot \vec{v}_2 + 2 \vec{v}_1 \cdot \vec{v}_2 \left( \vec{S}_1 \cdot \vec{v}_1 \right)^2 - 2 \vec{S}_1 \cdot \vec{S}_1 \vec{v}_1 \cdot \vec{v}_1 \vec{v}_1 \cdot \vec{v}_2 \right) \right) \Bigg\}$$

$$\{\text{DiagS1S1}[2, 2, 9],$$

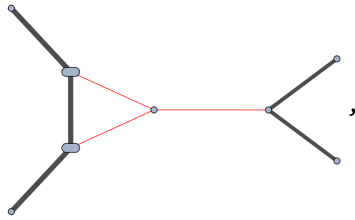

$$G^2 \left( \frac{1}{r^2} \left( 2 \left( \hat{n} \times \vec{S}_1 \cdot \vec{v}_1 \right)^2 + 4 \hat{n} \times \vec{S}_1 \cdot \vec{a}_1 \hat{n} \times \vec{S}_1 \cdot \vec{v}_1 + 2 \left( \hat{n} \times \vec{S}_1 \cdot \vec{a}_1 \right)^2 + 2 \left( \frac{1}{\vec{S}_1} \cdot \vec{v}_1 \right)^2 + \right. \right. \\ \left. \left. 2 \left( \vec{S}_1 \cdot \vec{a}_1 \right)^2 - 2 \vec{a}_1 \cdot \vec{a}_1 \vec{S}_1 \cdot \vec{S}_1 + 4 \frac{1}{\vec{S}_1} \cdot \vec{a}_1 \vec{S}_1 \cdot \vec{v}_1 - 4 \vec{S}_1 \cdot \frac{1}{\vec{S}_1} \vec{v}_1 \cdot \vec{a}_1 - 2 \frac{1}{\vec{S}_1} \cdot \frac{1}{\vec{S}_1} \vec{v}_1 \cdot \vec{v}_1 \right) + \frac{1}{r^3} \right. \\ \left( -4 \hat{n} \times \vec{S}_1 \cdot \vec{v}_1 \frac{1}{\vec{S}_1} \times \vec{v}_1 \cdot \vec{v}_2 - 4 \hat{n} \times \vec{S}_1 \cdot \vec{v}_1 \vec{S}_1 \times \vec{a}_1 \cdot \vec{v}_2 - 4 \hat{n} \times \vec{S}_1 \cdot \vec{v}_1 \vec{S}_1 \times \vec{v}_1 \cdot \vec{a}_1 - 4 \hat{n} \times \vec{S}_1 \cdot \vec{v}_1 \vec{S}_1 \times \vec{v}_1 \cdot \vec{v}_2 - \right. \\ \left. 4 \hat{n} \times \vec{S}_1 \cdot \vec{a}_1 \vec{S}_1 \times \vec{v}_1 \cdot \vec{v}_2 - 8 \hat{n} \times \vec{S}_1 \cdot \vec{v}_1 \hat{n} \times \vec{S}_1 \cdot \vec{v}_1 \hat{n} \cdot \vec{v}_1 - 8 \hat{n} \times \vec{S}_1 \cdot \vec{a}_1 \hat{n} \times \vec{S}_1 \cdot \vec{v}_1 \hat{n} \cdot \vec{v}_1 + 16 \hat{n} \times \vec{S}_1 \cdot \vec{v}_1 \hat{n} \times \vec{S}_1 \cdot \vec{v}_1 \hat{n} \cdot \vec{v}_2 + \right. \\ \left. 16 \hat{n} \times \vec{S}_1 \cdot \vec{a}_1 \hat{n} \times \vec{S}_1 \cdot \vec{v}_1 \hat{n} \cdot \vec{v}_2 - 4 \hat{n} \cdot \vec{v}_1 \frac{1}{\vec{S}_1} \cdot \vec{v}_1 \vec{S}_1 \cdot \vec{v}_1 + 8 \hat{n} \cdot \vec{v}_2 \frac{1}{\vec{S}_1} \cdot \vec{v}_1 \vec{S}_1 \cdot \vec{v}_1 - 4 \hat{n} \cdot \vec{v}_1 \vec{S}_1 \cdot \vec{a}_1 \vec{S}_1 \cdot \vec{v}_1 + 8 \hat{n} \cdot \vec{v}_2 \right. \\ \left. \vec{S}_1 \cdot \vec{a}_1 \vec{S}_1 \cdot \vec{v}_1 + 4 \hat{n} \cdot \vec{v}_1 \vec{S}_1 \cdot \vec{S}_1 \vec{v}_1 \cdot \vec{a}_1 - 8 \hat{n} \cdot \vec{v}_2 \vec{S}_1 \cdot \vec{S}_1 \vec{v}_1 \cdot \vec{a}_1 + 4 \hat{n} \cdot \vec{v}_1 \vec{S}_1 \cdot \frac{1}{\vec{S}_1} \vec{v}_1 \cdot \vec{v}_1 - 8 \hat{n} \cdot \vec{v}_2 \vec{S}_1 \cdot \frac{1}{\vec{S}_1} \vec{v}_1 \cdot \vec{v}_1 \right) + \\ \left. \frac{1}{r^4} \left( 9 \left( \hat{n} \cdot \vec{v}_1 \right)^2 \left( \hat{n} \times \vec{S}_1 \cdot \vec{v}_1 \right)^2 - 48 \hat{n} \cdot \vec{v}_1 \hat{n} \cdot \vec{v}_2 \left( \hat{n} \times \vec{S}_1 \cdot \vec{v}_1 \right)^2 - 3 \vec{v}_1 \cdot \vec{v}_1 \left( \hat{n} \times \vec{S}_1 \cdot \vec{v}_1 \right)^2 + \right. \right. \\ \left. \left. 8 \vec{v}_1 \cdot \vec{v}_2 \left( \hat{n} \times \vec{S}_1 \cdot \vec{v}_1 \right)^2 + 16 \vec{S}_1 \times \vec{v}_1 \cdot \vec{v}_2 \hat{n} \cdot \vec{v}_1 \hat{n} \times \vec{S}_1 \cdot \vec{v}_1 + 3 \left( \hat{n} \cdot \vec{v}_1 \right)^2 \left( \vec{S}_1 \cdot \vec{v}_1 \right)^2 - \right. \right. \\ \left. \left. 16 \hat{n} \cdot \vec{v}_1 \hat{n} \cdot \vec{v}_2 \left( \vec{S}_1 \cdot \vec{v}_1 \right)^2 + \vec{S}_1 \cdot \vec{S}_1 \left( \vec{v}_1 \cdot \vec{v}_1 \right)^2 - \left( \vec{S}_1 \cdot \vec{v}_1 \right)^2 \vec{v}_1 \cdot \vec{v}_1 - 3 \left( \hat{n} \cdot \vec{v}_1 \right)^2 \vec{S}_1 \cdot \vec{S}_1 \vec{v}_1 \cdot \vec{v}_1 + \right. \right. \\ \left. \left. 16 \hat{n} \cdot \vec{v}_1 \hat{n} \cdot \vec{v}_2 \vec{S}_1 \cdot \vec{S}_1 \vec{v}_1 \cdot \vec{v}_1 + 4 \left( \vec{S}_1 \cdot \vec{v}_1 \right)^2 \vec{v}_1 \cdot \vec{v}_2 - 4 \vec{S}_1 \cdot \vec{S}_1 \vec{v}_1 \cdot \vec{v}_1 \vec{v}_1 \cdot \vec{v}_2 \right) \right) m_2 \Bigg\}$$

$$\{\text{DiagS1S1}[2, 2, 10],$$

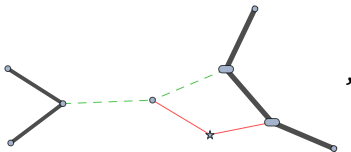

$$G^2 \left( \frac{1}{r^2} \left( -4 \hat{n} \times \vec{S_1} \cdot \vec{v_1} \hat{n} \times \vec{S_1} \cdot \vec{v_2} - 4 \hat{n} \times \vec{S_1} \cdot \vec{a_1} \hat{n} \times \vec{S_1} \cdot \vec{v_2} - 4 \hat{n} \times \vec{S_1} \cdot \vec{v_1} \hat{n} \times \vec{S_1} \cdot \vec{a_2} - 4 \hat{n} \times \vec{S_1} \cdot \vec{a_1} \hat{n} \times \vec{S_1} \cdot \vec{a_2} - \right. \right. \\ \left. \left. 6 \hat{n} \cdot \vec{v_1} \hat{n} \cdot \vec{v_2} \vec{S_1} \cdot \vec{S_1} + 6 \hat{n} \cdot \vec{S_1} \hat{n} \cdot \vec{v_2} \vec{S_1} \cdot \vec{a_1} + 6 \hat{n} \cdot \vec{S_1} \hat{n} \cdot \vec{v_2} \vec{S_1} \cdot \vec{v_1} - 2 \vec{S_1} \cdot \vec{v_1} \vec{S_1} \cdot \vec{v_2} - 6 \hat{n} \cdot \vec{a_2} \hat{n} \cdot \vec{v_1} \vec{S_1} \cdot \vec{S_1} - \right. \right. \\ \left. \left. 6 \hat{n} \cdot \vec{a_1} \hat{n} \cdot \vec{v_2} \vec{S_1} \cdot \vec{S_1} + 2 \vec{a_1} \cdot \vec{v_2} \vec{S_1} \cdot \vec{S_1} + 6 \hat{n} \cdot \vec{a_2} \hat{n} \cdot \vec{S_1} \vec{S_1} \cdot \vec{a_1} - 2 \vec{S_1} \cdot \vec{a_1} \vec{S_1} \cdot \vec{a_2} - 6 \hat{n} \cdot \vec{a_1} \hat{n} \cdot \vec{a_2} \vec{S_1} \cdot \vec{S_1} + \right. \right. \\ \left. \left. 6 \hat{n} \cdot \vec{a_1} \hat{n} \cdot \vec{a_2} \vec{S_1} \cdot \vec{v_1} - 6 \hat{n} \cdot \vec{a_1} \hat{n} \cdot \vec{a_2} \vec{S_1} \cdot \vec{v_2} - 6 \hat{n} \cdot \vec{a_1} \hat{n} \cdot \vec{a_2} \vec{S_1} \cdot \vec{v_1} \cdot \vec{v_2} - 6 \hat{n} \cdot \vec{a_1} \hat{n} \cdot \vec{a_2} \vec{S_1} \cdot \vec{v_1} \cdot \vec{v_2} \right) \right)$$

[illegible]

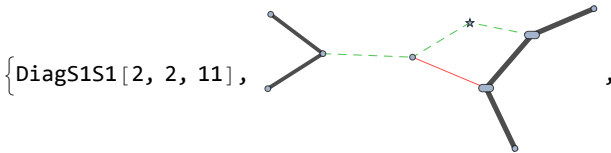

$$\begin{aligned} G^2 & \left( \frac{1}{r^2} \left( -12 \hat{n} \times \vec{S_1} \cdot \vec{v_1} \hat{n} \times \vec{S_1} \cdot \vec{v_2} - 12 \hat{n} \times \vec{S_1} \cdot \vec{a_1} \hat{n} \times \vec{S_1} \cdot \vec{v_2} - 12 \hat{n} \times \vec{S_1} \cdot \vec{a_2} \hat{n} \times \vec{S_1} \cdot \vec{v_1} - 2 \hat{n} \cdot \vec{v_1} \hat{n} \cdot \vec{v_2} \vec{S_1} \cdot \vec{S_1} + \right. \right. \\ & 2 \hat{n} \cdot \vec{S_1} \hat{n} \cdot \vec{v_2} \vec{S_1} \cdot \vec{a_1} + 2 \hat{n} \cdot \vec{a_2} \hat{n} \cdot \vec{S_1} \vec{S_1} \cdot \vec{v_1} + 2 \hat{n} \cdot \vec{S_1} \hat{n} \cdot \vec{v_2} \vec{S_1} \cdot \vec{v_1} - 6 \vec{S_1} \cdot \vec{v_1} \vec{S_1} \cdot \vec{v_2} - 2 \hat{n} \cdot \vec{a_2} \hat{n} \cdot \vec{v_1} \vec{S_1} \cdot \vec{S_1} - \\ & \left. \left. 2 \hat{n} \cdot \vec{a_1} \hat{n} \cdot \vec{v_2} \vec{S_1} \cdot \vec{S_1} + 6 \vec{a_1} \cdot \vec{v_2} \vec{S_1} \cdot \vec{S_1} - 6 \vec{S_1} \cdot \vec{v_1} \vec{S_1} \cdot \vec{a_2} - 6 \vec{S_1} \cdot \vec{a_1} \vec{S_1} \cdot \vec{v_2} + 6 \vec{S_1} \cdot \vec{S_1} \vec{v_1} \cdot \vec{a_2} + 6 \vec{S_1} \cdot \vec{S_1} \vec{v_1} \cdot \vec{v_2} \right) + \right. \\ & \left. \frac{1}{r^3} \left( 4 \hat{n} \cdot \vec{a_2} \left( \hat{n} \times \vec{S_1} \cdot \vec{v_1} \right)^2 + 6 \vec{S_1} \times \vec{v_1} \cdot \vec{v_2} \hat{n} \times \vec{S_1} \cdot \vec{v_1} - 2 \vec{S_1} \times \vec{a_1} \cdot \vec{v_2} \hat{n} \times \vec{S_1} \cdot \vec{v_1} + 2 \vec{S_1} \times \vec{v_1} \cdot \vec{a_2} \hat{n} \times \vec{S_1} \cdot \vec{v_1} + \right. \right. \\ & 36 \hat{n} \times \vec{S_1} \cdot \vec{v_2} \hat{n} \cdot \vec{v_1} \hat{n} \times \vec{S_1} \cdot \vec{v_1} + 12 \hat{n} \times \vec{S_1} \cdot \vec{a_2} \hat{n} \cdot \vec{v_1} \hat{n} \times \vec{S_1} \cdot \vec{v_1} - 48 \hat{n} \times \vec{S_1} \cdot \vec{v_2} \hat{n} \cdot \vec{v_2} \hat{n} \times \vec{S_1} \cdot \vec{v_1} + \\ & \left. \left. 4 \hat{n} \times \vec{S_1} \cdot \vec{a_1} \hat{n} \cdot \vec{v_2} \hat{n} \times \vec{S_1} \cdot \vec{v_1} + 2 \hat{n} \cdot \vec{a_2} \left( \vec{S_1} \cdot \vec{v_1} \right)^2 + 4 \hat{n} \times \vec{S_1} \cdot \vec{v_2} \vec{S_1} \times \vec{v_1} \cdot \vec{a_1} + 6 \hat{n} \times \vec{S_1} \cdot \vec{v_1} \vec{S_1} \times \vec{v_1} \cdot \vec{v_2} + \right. \right. \end{aligned}$$



$$2 \vec{S}_1 \cdot \vec{v}_1 \vec{S}_1 \cdot \vec{v}_2 \vec{v}_1 \cdot \vec{v}_2 + 2 \left( \vec{S}_1 \cdot \vec{v}_1 \right)^2 \vec{v}_2 \cdot \vec{v}_2 - 2 \vec{S}_1 \cdot \vec{S}_1 \vec{v}_1 \cdot \vec{v}_1 \vec{v}_2 \cdot \vec{v}_2 \Bigg) m_2 \Bigg\}$$

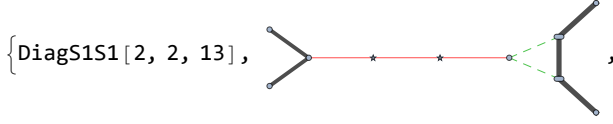

$$\begin{aligned} G^2 \Bigg( & \frac{1}{r} \left( \frac{1}{6} \hat{n} \cdot \vec{a}_2 \left( \hat{n} \cdot \vec{S}_1 \right)^2 - \frac{1}{6} \vec{S}_1 \cdot \vec{a}_2 \hat{n} \cdot \vec{S}_1 + \frac{1}{6} \hat{n} \cdot \vec{S}_1 \hat{n} \cdot \vec{a}_2 \hat{n} \cdot \vec{S}_1 - \right. \\ & \left. \frac{1}{3} \hat{n} \cdot \vec{a}_2 \vec{S}_1 \cdot \vec{S}_1 - \frac{1}{12} \hat{n} \cdot \vec{S}_1 \vec{S}_1 \cdot \vec{a}_2 - \frac{1}{3} \hat{n} \cdot \vec{a}_2 \vec{S}_1 \cdot \vec{S}_1 - \frac{1}{12} \hat{n} \cdot \vec{S}_1 \vec{S}_1 \cdot \vec{a}_2 \right) + \frac{1}{r^2} \\ & \left( \frac{2}{3} (\hat{n} \cdot \vec{v}_2)^2 \left( \hat{n} \cdot \vec{S}_1 \right)^2 - \frac{1}{6} \vec{v}_2 \cdot \vec{v}_2 \left( \hat{n} \cdot \vec{S}_1 \right)^2 - \frac{4}{3} \hat{n} \cdot \vec{a}_2 \hat{n} \cdot \vec{S}_1 \hat{n} \cdot \vec{v}_1 \hat{n} \cdot \vec{S}_1 - \frac{2}{3} \hat{n} \cdot \vec{v}_2 \vec{S}_1 \cdot \vec{v}_2 \hat{n} \cdot \vec{S}_1 + \right. \\ & \frac{1}{3} \hat{n} \cdot \vec{v}_1 \vec{S}_1 \cdot \vec{a}_2 \hat{n} \cdot \vec{S}_1 + \frac{1}{3} \hat{n} \cdot \vec{a}_2 \vec{S}_1 \cdot \vec{v}_1 \hat{n} \cdot \vec{S}_1 + \frac{1}{3} \hat{n} \cdot \vec{S}_1 \vec{v}_1 \cdot \vec{a}_2 \hat{n} \cdot \vec{S}_1 - \frac{1}{3} \hat{n} \cdot \vec{a}_1 \hat{n} \cdot \vec{a}_2 (\hat{n} \cdot \vec{S}_1)^2 + \\ & \frac{2}{3} \hat{n} \cdot \vec{S}_1 \hat{n} \cdot \vec{S}_1 (\hat{n} \cdot \vec{v}_2)^2 + \frac{1}{6} \left( \vec{S}_1 \cdot \vec{v}_2 \right)^2 - \frac{2}{3} (\hat{n} \cdot \vec{v}_2)^2 \vec{S}_1 \cdot \vec{S}_1 + \frac{1}{3} \hat{n} \cdot \vec{S}_1 \hat{n} \cdot \vec{v}_1 \vec{S}_1 \cdot \vec{a}_2 + \frac{1}{3} \hat{n} \cdot \vec{a}_2 \hat{n} \cdot \vec{S}_1 \vec{S}_1 \cdot \vec{v}_1 - \\ & \frac{1}{3} \hat{n} \cdot \vec{S}_1 \hat{n} \cdot \vec{v}_2 \vec{S}_1 \cdot \vec{v}_2 + \frac{1}{12} (\hat{n} \cdot \vec{S}_1)^2 \vec{a}_1 \cdot \vec{a}_2 + \frac{4}{3} \hat{n} \cdot \vec{a}_2 \hat{n} \cdot \vec{v}_1 \vec{S}_1 \cdot \vec{S}_1 - \frac{2}{3} (\hat{n} \cdot \vec{v}_2)^2 \vec{S}_1 \cdot \vec{S}_1 + \\ & \frac{1}{6} \hat{n} \cdot \vec{a}_2 \hat{n} \cdot \vec{S}_1 \vec{S}_1 \cdot \vec{a}_1 + \frac{1}{6} \hat{n} \cdot \vec{a}_1 \hat{n} \cdot \vec{S}_1 \vec{S}_1 \cdot \vec{a}_2 - \frac{1}{6} \vec{S}_1 \cdot \vec{v}_1 \vec{S}_1 \cdot \vec{a}_2 - \frac{1}{12} \vec{S}_1 \cdot \vec{a}_1 \vec{S}_1 \cdot \vec{a}_2 + \\ & \frac{1}{3} \hat{n} \cdot \vec{a}_1 \hat{n} \cdot \vec{a}_2 \vec{S}_1 \cdot \vec{S}_1 - \frac{1}{6} \vec{a}_1 \cdot \vec{a}_2 \vec{S}_1 \cdot \vec{S}_1 - \frac{1}{6} \vec{S}_1 \cdot \vec{a}_2 \vec{S}_1 \cdot \vec{v}_1 - \frac{1}{3} \hat{n} \cdot \vec{S}_1 \hat{n} \cdot \vec{v}_2 \vec{S}_1 \cdot \vec{v}_2 + \\ & \left. \frac{1}{6} \vec{S}_1 \cdot \vec{v}_2 \vec{S}_1 \cdot \vec{v}_2 - \frac{2}{3} \vec{S}_1 \cdot \vec{S}_1 \vec{v}_1 \cdot \vec{a}_2 - \frac{1}{6} \hat{n} \cdot \vec{S}_1 \hat{n} \cdot \vec{S}_1 \vec{v}_2 \cdot \vec{v}_2 + \frac{1}{3} \vec{S}_1 \cdot \vec{S}_1 \vec{v}_2 \cdot \vec{v}_2 + \frac{1}{3} \vec{S}_1 \cdot \vec{S}_1 \vec{v}_2 \cdot \vec{v}_2 \right) + \\ & \frac{1}{r^3} \left( 2 \hat{n} \cdot \vec{a}_2 (\hat{n} \cdot \vec{v}_1)^2 (\hat{n} \cdot \vec{S}_1)^2 - 2 \hat{n} \cdot \vec{a}_1 (\hat{n} \cdot \vec{v}_2)^2 (\hat{n} \cdot \vec{S}_1)^2 + \frac{2}{3} \hat{n} \cdot \vec{v}_2 \vec{a}_1 \cdot \vec{v}_2 (\hat{n} \cdot \vec{S}_1)^2 - \right. \\ & \frac{2}{3} \hat{n} \cdot \vec{v}_1 \vec{v}_1 \cdot \vec{a}_2 (\hat{n} \cdot \vec{S}_1)^2 - \frac{1}{3} \hat{n} \cdot \vec{a}_2 \vec{v}_1 \cdot \vec{v}_1 (\hat{n} \cdot \vec{S}_1)^2 + \frac{1}{3} \hat{n} \cdot \vec{a}_1 \vec{v}_2 \cdot \vec{v}_2 (\hat{n} \cdot \vec{S}_1)^2 - 8 \hat{n} \cdot \vec{S}_1 \hat{n} \cdot \vec{v}_1 (\hat{n} \cdot \vec{v}_2)^2 \hat{n} \cdot \vec{S}_1 + \\ & \frac{4}{3} (\hat{n} \cdot \vec{v}_2)^2 \vec{S}_1 \cdot \vec{v}_1 \hat{n} \cdot \vec{S}_1 + \frac{8}{3} \hat{n} \cdot \vec{v}_1 \hat{n} \cdot \vec{v}_2 \vec{S}_1 \cdot \vec{v}_2 \hat{n} \cdot \vec{S}_1 + \frac{2}{3} (\hat{n} \cdot \vec{v}_2)^2 \vec{S}_1 \cdot \vec{a}_1 \hat{n} \cdot \vec{S}_1 - \\ & \frac{2}{3} (\hat{n} \cdot \vec{v}_1)^2 \vec{S}_1 \cdot \vec{a}_2 \hat{n} \cdot \vec{S}_1 - \frac{4}{3} \hat{n} \cdot \vec{a}_2 \hat{n} \cdot \vec{v}_1 \vec{S}_1 \cdot \vec{v}_1 \hat{n} \cdot \vec{S}_1 + \frac{4}{3} \hat{n} \cdot \vec{a}_1 \hat{n} \cdot \vec{v}_2 \vec{S}_1 \cdot \vec{v}_2 \hat{n} \cdot \vec{S}_1 - \\ & \frac{1}{3} \vec{a}_1 \cdot \vec{v}_2 \vec{S}_1 \cdot \vec{v}_2 \hat{n} \cdot \vec{S}_1 + \frac{1}{3} \vec{S}_1 \cdot \vec{v}_1 \vec{v}_1 \cdot \vec{a}_2 \hat{n} \cdot \vec{S}_1 + \frac{1}{6} \vec{S}_1 \cdot \vec{a}_2 \vec{v}_1 \cdot \vec{v}_1 \hat{n} \cdot \vec{S}_1 + \frac{8}{3} \hat{n} \cdot \vec{S}_1 \hat{n} \cdot \vec{v}_2 \vec{v}_1 \cdot \vec{v}_2 \hat{n} \cdot \vec{S}_1 - \\ & \frac{2}{3} \vec{S}_1 \cdot \vec{v}_2 \vec{v}_1 \cdot \vec{v}_2 \hat{n} \cdot \vec{S}_1 + \frac{4}{3} \hat{n} \cdot \vec{S}_1 \hat{n} \cdot \vec{v}_1 \vec{v}_2 \cdot \vec{v}_2 \hat{n} \cdot \vec{S}_1 - \frac{1}{3} \vec{S}_1 \cdot \vec{v}_1 \vec{v}_2 \cdot \vec{v}_2 \hat{n} \cdot \vec{S}_1 - \frac{1}{6} \vec{S}_1 \cdot \vec{a}_1 \vec{v}_2 \cdot \vec{v}_2 \hat{n} \cdot \vec{S}_1 + \\ & \frac{1}{6} \hat{n} \cdot \vec{a}_2 (\vec{S}_1 \cdot \vec{v}_1)^2 - \frac{1}{6} \hat{n} \cdot \vec{a}_1 (\vec{S}_1 \cdot \vec{v}_2)^2 + \frac{16}{3} \hat{n} \cdot \vec{v}_1 (\hat{n} \cdot \vec{v}_2)^2 \vec{S}_1 \cdot \vec{S}_1 - \frac{4}{3} \hat{n} \cdot \vec{a}_2 (\hat{n} \cdot \vec{v}_1)^2 \vec{S}_1 \cdot \vec{S}_1 + \\ & \frac{4}{3} \hat{n} \cdot \vec{a}_1 (\hat{n} \cdot \vec{v}_2)^2 \vec{S}_1 \cdot \vec{S}_1 - \frac{2}{3} \hat{n} \cdot \vec{v}_2 \vec{a}_1 \cdot \vec{v}_2 \vec{S}_1 \cdot \vec{S}_1 + \frac{4}{3} \hat{n} \cdot \vec{S}_1 (\hat{n} \cdot \vec{v}_2)^2 \vec{S}_1 \cdot \vec{v}_1 - \frac{2}{3} \hat{n} \cdot \vec{v}_2 \vec{S}_1 \cdot \vec{v}_2 \vec{S}_1 \cdot \vec{v}_1 + \\ & \frac{1}{3} \hat{n} \cdot \vec{v}_1 \vec{S}_1 \cdot \vec{a}_2 \vec{S}_1 \cdot \vec{v}_1 + \frac{8}{3} \hat{n} \cdot \vec{S}_1 \hat{n} \cdot \vec{v}_1 \hat{n} \cdot \vec{v}_2 \vec{S}_1 \cdot \vec{v}_2 - \frac{2}{3} \hat{n} \cdot \vec{v}_2 \vec{S}_1 \cdot \vec{v}_1 \vec{S}_1 \cdot \vec{v}_2 - \frac{2}{3} \hat{n} \cdot \vec{v}_1 \vec{S}_1 \cdot \vec{v}_2 \vec{S}_1 \cdot \vec{v}_2 - \\ & \frac{1}{3} \hat{n} \cdot \vec{v}_2 \vec{S}_1 \cdot \vec{a}_1 \vec{S}_1 \cdot \vec{v}_2 + \frac{2}{3} \hat{n} \cdot \vec{v}_1 \vec{S}_1 \cdot \vec{S}_1 \vec{v}_1 \cdot \vec{a}_2 + \frac{1}{3} \hat{n} \cdot \vec{a}_2 \vec{S}_1 \cdot \vec{S}_1 \vec{v}_1 \cdot \vec{v}_1 - \frac{8}{3} \hat{n} \cdot \vec{v}_2 \vec{S}_1 \cdot \vec{S}_1 \vec{v}_1 \cdot \vec{v}_2 - \\ & \left. \frac{2}{3} \hat{n} \cdot \vec{S}_1 \vec{S}_1 \cdot \vec{v}_2 \vec{v}_1 \cdot \vec{v}_2 - \frac{4}{3} \hat{n} \cdot \vec{v}_1 \vec{S}_1 \cdot \vec{S}_1 \vec{v}_2 \cdot \vec{v}_2 - \frac{1}{3} \hat{n} \cdot \vec{a}_1 \vec{S}_1 \cdot \vec{S}_1 \vec{v}_2 \cdot \vec{v}_2 - \frac{1}{3} \hat{n} \cdot \vec{S}_1 \vec{S}_1 \cdot \vec{v}_1 \vec{v}_2 \cdot \vec{v}_2 \right) + \\ & \frac{1}{r^4} \left( 16 (\hat{n} \cdot \vec{v}_1)^2 (\hat{n} \cdot \vec{v}_2)^2 (\hat{n} \cdot \vec{S}_1)^2 + \frac{2}{3} (\vec{v}_1 \cdot \vec{v}_2)^2 (\hat{n} \cdot \vec{S}_1)^2 - 2 (\hat{n} \cdot \vec{v}_2)^2 \vec{v}_1 \cdot \vec{v}_1 (\hat{n} \cdot \vec{S}_1)^2 - \right. \\ & \left. 8 \hat{n} \cdot \vec{v}_1 \hat{n} \cdot \vec{v}_2 \vec{v}_1 \cdot \vec{v}_2 (\hat{n} \cdot \vec{S}_1)^2 - 2 (\hat{n} \cdot \vec{v}_1)^2 \vec{v}_2 \cdot \vec{v}_2 (\hat{n} \cdot \vec{S}_1)^2 + \frac{1}{3} \vec{v}_1 \cdot \vec{v}_1 \vec{v}_2 \cdot \vec{v}_2 (\hat{n} \cdot \vec{S}_1)^2 - \right. \end{aligned}$$

$$\begin{aligned}
& 8 \hat{n} \cdot \vec{v}_1 (\hat{n} \cdot \vec{v}_2)^2 \vec{S}_1 \cdot \vec{v}_1 \hat{n} \cdot \vec{S}_1 - 8 (\hat{n} \cdot \vec{v}_1)^2 \hat{n} \cdot \vec{v}_2 \vec{S}_1 \cdot \vec{v}_2 \hat{n} \cdot \vec{S}_1 + \frac{4}{3} \hat{n} \cdot \vec{v}_2 \vec{S}_1 \cdot \vec{v}_2 \vec{v}_1 \cdot \vec{v}_1 \hat{n} \cdot \vec{S}_1 + \\
& \frac{8}{3} \hat{n} \cdot \vec{v}_2 \vec{S}_1 \cdot \vec{v}_1 \vec{v}_1 \cdot \vec{v}_2 \hat{n} \cdot \vec{S}_1 + \frac{8}{3} \hat{n} \cdot \vec{v}_1 \vec{S}_1 \cdot \vec{v}_2 \vec{v}_1 \cdot \vec{v}_2 \hat{n} \cdot \vec{S}_1 + \frac{4}{3} \hat{n} \cdot \vec{v}_1 \vec{S}_1 \cdot \vec{v}_1 \vec{v}_2 \cdot \vec{v}_2 \hat{n} \cdot \vec{S}_1 + \\
& \frac{2}{3} (\hat{n} \cdot \vec{v}_2)^2 (\vec{S}_1 \cdot \vec{v}_1)^2 + \frac{2}{3} (\hat{n} \cdot \vec{v}_1)^2 (\vec{S}_1 \cdot \vec{v}_2)^2 - \frac{2}{3} \vec{S}_1 \cdot \vec{S}_1 (\vec{v}_1 \cdot \vec{v}_2)^2 - 8 (\hat{n} \cdot \vec{v}_1)^2 (\hat{n} \cdot \vec{v}_2)^2 \vec{S}_1 \cdot \vec{S}_1 + \\
& \frac{8}{3} \hat{n} \cdot \vec{v}_1 \hat{n} \cdot \vec{v}_2 \vec{S}_1 \cdot \vec{v}_1 \vec{S}_1 \cdot \vec{v}_2 - \frac{1}{6} (\vec{S}_1 \cdot \vec{v}_2)^2 \vec{v}_1 \cdot \vec{v}_1 + \frac{4}{3} (\hat{n} \cdot \vec{v}_2)^2 \vec{S}_1 \cdot \vec{S}_1 \vec{v}_1 \cdot \vec{v}_1 + \frac{16}{3} \hat{n} \cdot \vec{v}_1 \hat{n} \cdot \vec{v}_2 \vec{S}_1 \cdot \vec{S}_1 \vec{v}_1 \cdot \vec{v}_2 - \\
& \frac{2}{3} \vec{S}_1 \cdot \vec{v}_1 \vec{S}_1 \cdot \vec{v}_2 \vec{v}_1 \cdot \vec{v}_2 - \frac{1}{6} (\vec{S}_1 \cdot \vec{v}_1)^2 \vec{v}_2 \cdot \vec{v}_2 + \frac{4}{3} (\hat{n} \cdot \vec{v}_1)^2 \vec{S}_1 \cdot \vec{S}_1 \vec{v}_2 \cdot \vec{v}_2 - \frac{1}{3} \vec{S}_1 \cdot \vec{S}_1 \vec{v}_1 \cdot \vec{v}_1 \vec{v}_2 \cdot \vec{v}_2 \Big) m_2 \Big\}
\end{aligned}$$

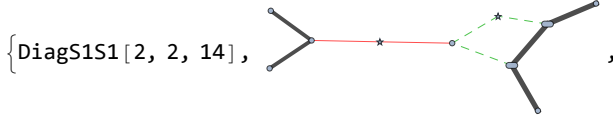

$$\begin{aligned}
& G^2 \left( \frac{1}{r} \left( -\frac{5}{6} \hat{n} \cdot \vec{a}_2 \left( \hat{n} \cdot \vec{S}_1 \right)^2 - \frac{5}{3} \hat{n} \cdot \vec{S}_1 \hat{n} \cdot \vec{v}_2 \hat{n} \cdot \vec{S}_1 + \frac{5}{6} \vec{S}_1 \cdot \vec{a}_2 \hat{n} \cdot \vec{S}_1 + \frac{5}{6} \vec{S}_1 \cdot \vec{v}_2 \hat{n} \cdot \vec{S}_1 - \frac{5}{6} \hat{n} \cdot \vec{S}_1 \hat{n} \cdot \vec{a}_2 \hat{n} \cdot \vec{S}_1 + \right. \right. \\
& \left. \frac{2}{3} \hat{n} \cdot \vec{a}_2 \vec{S}_1 \cdot \vec{S}_1 + \frac{4}{3} \hat{n} \cdot \vec{v}_2 \vec{S}_1 \cdot \vec{S}_1 + \frac{5}{6} \hat{n} \cdot \vec{S}_1 \vec{S}_1 \cdot \vec{v}_2 + \frac{5}{12} \hat{n} \cdot \vec{S}_1 \vec{S}_1 \cdot \vec{a}_2 + \frac{2}{3} \hat{n} \cdot \vec{a}_2 \vec{S}_1 \cdot \vec{S}_1 + \frac{5}{12} \hat{n} \cdot \vec{S}_1 \vec{S}_1 \cdot \vec{a}_2 \right) + \\
& \frac{1}{r^2} \left( -\frac{10}{3} (\hat{n} \cdot \vec{v}_2)^2 \left( \hat{n} \cdot \vec{S}_1 \right)^2 + \frac{20}{3} \hat{n} \cdot \vec{v}_1 \hat{n} \cdot \vec{v}_2 \left( \hat{n} \cdot \vec{S}_1 \right)^2 - \frac{5}{3} \vec{v}_1 \cdot \vec{v}_2 \left( \hat{n} \cdot \vec{S}_1 \right)^2 + \frac{5}{6} \vec{v}_2 \cdot \vec{v}_2 \left( \hat{n} \cdot \vec{S}_1 \right)^2 + \right. \\
& \frac{14}{3} \hat{n} \cdot \vec{a}_2 \hat{n} \cdot \vec{S}_1 \hat{n} \cdot \vec{v}_1 \hat{n} \cdot \vec{S}_1 + \frac{10}{3} \hat{n} \cdot \vec{a}_1 \hat{n} \cdot \vec{S}_1 \hat{n} \cdot \vec{v}_2 \hat{n} \cdot \vec{S}_1 - \frac{10}{3} \hat{n} \cdot \vec{v}_2 \vec{S}_1 \cdot \vec{v}_1 \hat{n} \cdot \vec{S}_1 - \frac{10}{3} \hat{n} \cdot \vec{v}_1 \vec{S}_1 \cdot \vec{v}_2 \hat{n} \cdot \vec{S}_1 + \\
& \frac{10}{3} \hat{n} \cdot \vec{v}_2 \vec{S}_1 \cdot \vec{v}_2 \hat{n} \cdot \vec{S}_1 - \frac{5}{6} \hat{n} \cdot \vec{S}_1 \vec{a}_1 \cdot \vec{v}_2 \hat{n} \cdot \vec{S}_1 + \frac{2}{3} \hat{n} \cdot \vec{v}_2 \vec{S}_1 \cdot \vec{a}_1 \hat{n} \cdot \vec{S}_1 - \frac{7}{6} \hat{n} \cdot \vec{v}_1 \vec{S}_1 \cdot \vec{a}_2 \hat{n} \cdot \vec{S}_1 - \\
& \frac{5}{3} \hat{n} \cdot \vec{a}_2 \vec{S}_1 \cdot \vec{v}_1 \hat{n} \cdot \vec{S}_1 - \frac{5}{6} \hat{n} \cdot \vec{a}_1 \vec{S}_1 \cdot \vec{v}_2 \hat{n} \cdot \vec{S}_1 - \frac{7}{6} \hat{n} \cdot \vec{S}_1 \vec{v}_1 \cdot \vec{a}_2 \hat{n} \cdot \vec{S}_1 + \frac{2}{3} \hat{n} \cdot \vec{a}_1 \hat{n} \cdot \vec{a}_2 \left( \hat{n} \cdot \vec{S}_1 \right)^2 - \\
& \frac{10}{3} \hat{n} \cdot \vec{S}_1 \hat{n} \cdot \vec{S}_1 (\hat{n} \cdot \vec{v}_2)^2 - \frac{5}{6} \left( \vec{S}_1 \cdot \vec{v}_2 \right)^2 + \frac{10}{3} \hat{n} \cdot \vec{S}_1 \hat{n} \cdot \vec{S}_1 \hat{n} \cdot \vec{v}_1 \hat{n} \cdot \vec{v}_2 + \frac{4}{3} (\hat{n} \cdot \vec{v}_2)^2 \vec{S}_1 \cdot \vec{S}_1 - \\
& \frac{8}{3} \hat{n} \cdot \vec{v}_1 \hat{n} \cdot \vec{v}_2 \vec{S}_1 \cdot \vec{S}_1 - \frac{7}{3} \hat{n} \cdot \vec{S}_1 \hat{n} \cdot \vec{v}_2 \vec{S}_1 \cdot \vec{a}_1 - \frac{7}{6} \hat{n} \cdot \vec{S}_1 \hat{n} \cdot \vec{v}_1 \vec{S}_1 \cdot \vec{a}_2 - \frac{5}{3} \hat{n} \cdot \vec{a}_2 \hat{n} \cdot \vec{S}_1 \vec{S}_1 \cdot \vec{v}_1 - \\
& \frac{5}{6} \hat{n} \cdot \vec{a}_1 \hat{n} \cdot \vec{S}_1 \vec{S}_1 \cdot \vec{v}_2 + \frac{5}{3} \vec{S}_1 \cdot \vec{v}_1 \vec{S}_1 \cdot \vec{v}_2 - \frac{7}{3} \hat{n} \cdot \vec{S}_1 \hat{n} \cdot \vec{v}_2 \vec{S}_1 \cdot \vec{v}_1 - \frac{5}{6} \hat{n} \cdot \vec{S}_1 \hat{n} \cdot \vec{v}_1 \vec{S}_1 \cdot \vec{v}_2 + \\
& \frac{5}{3} \hat{n} \cdot \vec{S}_1 \hat{n} \cdot \vec{v}_2 \vec{S}_1 \cdot \vec{v}_2 - \frac{1}{6} (\hat{n} \cdot \vec{S}_1)^2 \vec{a}_1 \cdot \vec{a}_2 - \frac{5}{3} \hat{n} \cdot \vec{a}_2 \hat{n} \cdot \vec{v}_1 \vec{S}_1 \cdot \vec{S}_1 - \frac{4}{3} \hat{n} \cdot \vec{a}_1 \hat{n} \cdot \vec{v}_2 \vec{S}_1 \cdot \vec{S}_1 + \\
& \frac{2}{3} \vec{a}_1 \cdot \vec{v}_2 \vec{S}_1 \cdot \vec{S}_1 + \frac{4}{3} (\hat{n} \cdot \vec{v}_2)^2 \vec{S}_1 \cdot \vec{S}_1 - \frac{4}{3} \hat{n} \cdot \vec{v}_1 \hat{n} \cdot \vec{v}_2 \vec{S}_1 \cdot \vec{S}_1 - \frac{5}{6} \hat{n} \cdot \vec{a}_2 \hat{n} \cdot \vec{S}_1 \vec{S}_1 \cdot \vec{a}_1 - \frac{1}{3} \vec{S}_1 \cdot \vec{v}_2 \vec{S}_1 \cdot \vec{a}_1 - \\
& \frac{1}{3} \hat{n} \cdot \vec{a}_1 \hat{n} \cdot \vec{S}_1 \vec{S}_1 \cdot \vec{a}_2 + \frac{5}{6} \vec{S}_1 \cdot \vec{v}_1 \vec{S}_1 \cdot \vec{a}_2 + \frac{5}{12} \vec{S}_1 \cdot \vec{a}_1 \vec{S}_1 \cdot \vec{a}_2 - \frac{1}{6} \hat{n} \cdot \vec{a}_1 \hat{n} \cdot \vec{a}_2 \vec{S}_1 \cdot \vec{S}_1 + \frac{1}{12} \vec{a}_1 \cdot \vec{a}_2 \vec{S}_1 \cdot \vec{S}_1 + \\
& \frac{2}{3} \hat{n} \cdot \vec{S}_1 \hat{n} \cdot \vec{v}_2 \vec{S}_1 \cdot \vec{v}_1 + \frac{5}{6} \vec{S}_1 \cdot \vec{a}_2 \vec{S}_1 \cdot \vec{v}_1 - \frac{1}{3} \vec{S}_1 \cdot \vec{v}_2 \vec{S}_1 \cdot \vec{v}_1 - \frac{5}{6} \hat{n} \cdot \vec{S}_1 \hat{n} \cdot \vec{v}_1 \vec{S}_1 \cdot \vec{v}_2 + \frac{5}{3} \hat{n} \cdot \vec{S}_1 \hat{n} \cdot \vec{v}_2 \vec{S}_1 \cdot \vec{v}_2 + \\
& \frac{7}{6} \vec{S}_1 \cdot \vec{a}_1 \vec{S}_1 \cdot \vec{v}_2 + \frac{7}{6} \vec{S}_1 \cdot \vec{v}_1 \vec{S}_1 \cdot \vec{v}_2 - \frac{5}{6} \vec{S}_1 \cdot \vec{v}_2 \vec{S}_1 \cdot \vec{v}_2 + \frac{5}{6} \vec{S}_1 \cdot \vec{S}_1 \vec{v}_1 \cdot \vec{a}_2 - \frac{5}{6} \hat{n} \cdot \vec{S}_1 \hat{n} \cdot \vec{S}_1 \vec{v}_1 \cdot \vec{v}_2 + \\
& \left. \frac{4}{3} \vec{S}_1 \cdot \vec{S}_1 \vec{v}_1 \cdot \vec{v}_2 + \frac{2}{3} \vec{S}_1 \cdot \vec{S}_1 \vec{v}_1 \cdot \vec{v}_2 + \frac{5}{6} \hat{n} \cdot \vec{S}_1 \hat{n} \cdot \vec{S}_1 \vec{v}_2 \cdot \vec{v}_2 - \frac{2}{3} \vec{S}_1 \cdot \vec{S}_1 \vec{v}_2 \cdot \vec{v}_2 - \frac{2}{3} \vec{S}_1 \cdot \vec{S}_1 \vec{v}_2 \cdot \vec{v}_2 \right) + \\
& \frac{1}{r^3} \left( -4 \hat{n} \cdot \vec{a}_2 (\hat{n} \cdot \vec{v}_1)^2 (\hat{n} \cdot \vec{S}_1)^2 + 4 \hat{n} \cdot \vec{a}_1 (\hat{n} \cdot \vec{v}_2)^2 (\hat{n} \cdot \vec{S}_1)^2 - \frac{9}{2} \hat{n} \cdot \vec{a}_1 \hat{n} \cdot \vec{v}_1 \hat{n} \cdot \vec{v}_2 (\hat{n} \cdot \vec{S}_1)^2 + \right. \\
& \frac{3}{4} \hat{n} \cdot \vec{v}_1 \vec{a}_1 \cdot \vec{v}_2 (\hat{n} \cdot \vec{S}_1)^2 - \frac{4}{3} \hat{n} \cdot \vec{v}_2 \vec{a}_1 \cdot \vec{v}_2 (\hat{n} \cdot \vec{S}_1)^2 + \hat{n} \cdot \vec{v}_2 \vec{v}_1 \cdot \vec{a}_1 (\hat{n} \cdot \vec{S}_1)^2 + \frac{4}{3} \hat{n} \cdot \vec{v}_1 \vec{v}_1 \cdot \vec{a}_2 (\hat{n} \cdot \vec{S}_1)^2 + \\
& \left. \frac{2}{3} \hat{n} \cdot \vec{a}_2 \vec{v}_1 \cdot \vec{v}_1 (\hat{n} \cdot \vec{S}_1)^2 + \frac{3}{4} \hat{n} \cdot \vec{a}_1 \vec{v}_1 \cdot \vec{v}_2 (\hat{n} \cdot \vec{S}_1)^2 - \frac{2}{3} \hat{n} \cdot \vec{a}_1 \vec{v}_2 \cdot \vec{v}_2 (\hat{n} \cdot \vec{S}_1)^2 + 28 \hat{n} \cdot \vec{S}_1 \hat{n} \cdot \vec{v}_1 (\hat{n} \cdot \vec{v}_2)^2 \hat{n} \cdot \vec{S}_1 - \right.
\end{aligned}$$



$$\begin{aligned} & \frac{1}{3} \vec{S}_1 \cdot \vec{S}_1 (\vec{v}_1 \cdot \vec{v}_2)^2 + 4 (\hat{n} \cdot \vec{S}_1)^2 (\hat{n} \cdot \vec{v}_2)^2 \vec{v}_1 \cdot \vec{v}_1 + \frac{1}{3} (\vec{S}_1 \cdot \vec{v}_2)^2 \vec{v}_1 \cdot \vec{v}_1 - \frac{2}{3} (\hat{n} \cdot \vec{v}_2)^2 \vec{S}_1 \cdot \vec{S}_1 \vec{v}_1 \cdot \vec{v}_1 + \\ & 5 \hat{n} \cdot \vec{S}_1 \hat{n} \cdot \vec{v}_2 \vec{S}_1 \cdot \vec{v}_1 \vec{v}_1 \cdot \vec{v}_1 - \frac{8}{3} \hat{n} \cdot \vec{S}_1 \hat{n} \cdot \vec{v}_2 \vec{S}_1 \cdot \vec{v}_2 \vec{v}_1 \cdot \vec{v}_1 - \frac{5}{4} \vec{S}_1 \cdot \vec{v}_1 \vec{S}_1 \cdot \vec{v}_2 \vec{v}_1 \cdot \vec{v}_1 - 2 (\hat{n} \times \vec{S}_1 \cdot \vec{v}_1)^2 \vec{v}_1 \cdot \vec{v}_2 - \\ & 2 (\vec{S}_1 \cdot \vec{v}_1)^2 \vec{v}_1 \cdot \vec{v}_2 - \frac{28}{3} \hat{n} \cdot \vec{S}_1 \hat{n} \cdot \vec{v}_2 \vec{S}_1 \cdot \vec{v}_1 \vec{v}_1 \cdot \vec{v}_2 + \frac{7}{3} \vec{S}_1 \cdot \vec{v}_1 \vec{S}_1 \cdot \vec{v}_2 \vec{v}_1 \cdot \vec{v}_2 + \frac{5}{4} (\hat{n} \cdot \vec{S}_1)^2 \vec{v}_1 \cdot \vec{v}_1 \vec{v}_1 \cdot \vec{v}_2 + \\ & \vec{S}_1 \cdot \vec{S}_1 \vec{v}_1 \cdot \vec{v}_1 \vec{v}_1 \cdot \vec{v}_2 + \frac{5}{6} (\vec{S}_1 \cdot \vec{v}_1)^2 \vec{v}_2 \cdot \vec{v}_2 - \frac{2}{3} (\hat{n} \cdot \vec{S}_1)^2 \vec{v}_1 \cdot \vec{v}_1 \vec{v}_2 \cdot \vec{v}_2 + \frac{1}{6} \vec{S}_1 \cdot \vec{S}_1 \vec{v}_1 \cdot \vec{v}_1 \vec{v}_2 \cdot \vec{v}_2 \Big) m_2 \} \end{aligned}$$

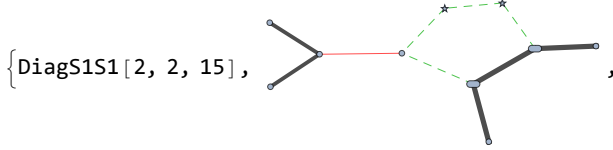

$$\begin{aligned} G^2 m_2 \Bigg( & \frac{7}{12} \left( \hat{n} \cdot \vec{S}_1 \right)^2 - \frac{23}{36} \vec{S}_1 \cdot \vec{S}_1 + \frac{1}{r} \left( -\frac{7}{6} \hat{n} \cdot \vec{S}_1 \hat{n} \cdot \vec{a}_1 \hat{n} \cdot \vec{S}_1 + \frac{7}{6} \hat{n} \cdot \vec{S}_1 \hat{n} \cdot \vec{a}_2 \hat{n} \cdot \vec{S}_1 + \frac{4}{3} \vec{S}_1 \cdot \vec{a}_1 \hat{n} \cdot \vec{S}_1 - \frac{7}{12} \vec{S}_1 \cdot \vec{a}_2 \hat{n} \cdot \vec{S}_1 - \right. \\ & \frac{7}{3} \hat{n} \cdot \vec{S}_1 \hat{n} \cdot \vec{S}_1 \hat{n} \cdot \vec{v}_1 + \frac{7}{3} \hat{n} \cdot \vec{S}_1 \hat{n} \cdot \vec{S}_1 \hat{n} \cdot \vec{v}_2 + \frac{2}{3} \hat{n} \cdot \vec{v}_1 \vec{S}_1 \cdot \vec{S}_1 - \frac{2}{3} \hat{n} \cdot \vec{v}_2 \vec{S}_1 \cdot \vec{S}_1 - \frac{1}{3} \hat{n} \cdot \vec{S}_1 \vec{S}_1 \cdot \vec{v}_1 - \frac{7}{6} \hat{n} \cdot \vec{S}_1 \vec{S}_1 \cdot \vec{v}_2 + \\ & \left. \frac{8}{3} \hat{n} \cdot \vec{S}_1 \vec{S}_1 \cdot \vec{v}_1 - \frac{7}{6} \hat{n} \cdot \vec{S}_1 \vec{S}_1 \cdot \vec{v}_2 + \frac{1}{3} \hat{n} \cdot \vec{a}_1 \vec{S}_1 \cdot \vec{S}_1 - \frac{1}{3} \hat{n} \cdot \vec{a}_2 \vec{S}_1 \cdot \vec{S}_1 - \frac{1}{6} \hat{n} \cdot \vec{S}_1 \vec{S}_1 \cdot \vec{a}_1 - \frac{7}{12} \hat{n} \cdot \vec{S}_1 \vec{S}_1 \cdot \vec{a}_2 \right) + \frac{1}{r^2} \\ & \left( 3 \left( \hat{n} \times \vec{S}_1 \cdot \vec{v}_1 \right)^2 + \frac{3}{2} \hat{n} \times \vec{S}_1 \cdot \vec{a}_1 \hat{n} \times \vec{S}_1 \cdot \vec{v}_1 + \frac{3}{4} \left( \hat{n} \times \vec{S}_1 \cdot \vec{a}_1 \right)^2 - \frac{13}{12} \left( \hat{n} \cdot \vec{a}_1 \right)^2 \left( \hat{n} \cdot \vec{S}_1 \right)^2 + \frac{4}{3} \hat{n} \cdot \vec{a}_1 \hat{n} \cdot \vec{a}_2 \left( \hat{n} \cdot \vec{S}_1 \right)^2 - \right. \\ & \frac{13}{3} \left( \hat{n} \cdot \vec{S}_1 \right)^2 \left( \hat{n} \cdot \vec{v}_1 \right)^2 + \frac{41}{6} \hat{n} \cdot \vec{S}_1 \hat{n} \cdot \vec{S}_1 \left( \hat{n} \cdot \vec{v}_1 \right)^2 + \frac{14}{3} \hat{n} \cdot \vec{S}_1 \hat{n} \cdot \vec{S}_1 \left( \hat{n} \cdot \vec{v}_2 \right)^2 + \frac{8}{3} \left( \vec{S}_1 \cdot \vec{v}_1 \right)^2 + \frac{2}{3} \left( \vec{S}_1 \cdot \vec{a}_1 \right)^2 + \\ & \frac{3}{2} \hat{n} \times \vec{S}_1 \cdot \vec{a}_1 \hat{n} \times \vec{S}_1 \cdot \vec{v}_1 - \frac{3}{2} \hat{n} \times \vec{S}_1 \cdot \vec{v}_1 \hat{n} \times \vec{S}_1 \cdot \vec{v}_1 - \frac{13}{3} \hat{n} \cdot \vec{S}_1 \hat{n} \cdot \vec{a}_1 \hat{n} \cdot \vec{S}_1 \hat{n} \cdot \vec{v}_1 + \frac{8}{3} \hat{n} \cdot \vec{S}_1 \hat{n} \cdot \vec{a}_2 \hat{n} \cdot \vec{S}_1 \hat{n} \cdot \vec{v}_1 + \\ & \frac{8}{3} \hat{n} \cdot \vec{S}_1 \hat{n} \cdot \vec{a}_1 \hat{n} \cdot \vec{S}_1 \hat{n} \cdot \vec{v}_2 + \frac{16}{3} \left( \hat{n} \cdot \vec{S}_1 \right)^2 \hat{n} \cdot \vec{v}_1 \hat{n} \cdot \vec{v}_2 - 12 \hat{n} \cdot \vec{S}_1 \hat{n} \cdot \vec{S}_1 \hat{n} \cdot \vec{v}_1 \hat{n} \cdot \vec{v}_2 + \frac{16}{3} \left( \hat{n} \cdot \vec{v}_1 \right)^2 \vec{S}_1 \cdot \vec{S}_1 - \\ & \frac{10}{3} \hat{n} \cdot \vec{v}_1 \hat{n} \cdot \vec{v}_2 \vec{S}_1 \cdot \vec{S}_1 - \frac{13}{6} \hat{n} \cdot \vec{S}_1 \hat{n} \cdot \vec{v}_1 \vec{S}_1 \cdot \vec{a}_1 + \frac{7}{3} \hat{n} \cdot \vec{S}_1 \hat{n} \cdot \vec{v}_2 \vec{S}_1 \cdot \vec{a}_1 - \frac{2}{3} \hat{n} \cdot \vec{S}_1 \hat{n} \cdot \vec{v}_1 \vec{S}_1 \cdot \vec{a}_2 + \\ & \frac{5}{6} \hat{n} \cdot \vec{a}_1 \hat{n} \cdot \vec{S}_1 \vec{S}_1 \cdot \vec{v}_1 - \frac{2}{3} \hat{n} \cdot \vec{a}_2 \hat{n} \cdot \vec{S}_1 \vec{S}_1 \cdot \vec{v}_1 - \frac{8}{3} \hat{n} \cdot \vec{S}_1 \hat{n} \cdot \vec{v}_1 \vec{S}_1 \cdot \vec{v}_1 + \frac{10}{3} \hat{n} \cdot \vec{S}_1 \hat{n} \cdot \vec{v}_2 \vec{S}_1 \cdot \vec{v}_1 - \\ & \frac{2}{3} \hat{n} \cdot \vec{a}_1 \hat{n} \cdot \vec{S}_1 \vec{S}_1 \cdot \vec{v}_2 - \frac{8}{3} \hat{n} \cdot \vec{S}_1 \hat{n} \cdot \vec{v}_1 \vec{S}_1 \cdot \vec{v}_2 - \frac{5}{3} \vec{S}_1 \cdot \vec{v}_1 \vec{S}_1 \cdot \vec{v}_2 - \frac{19}{6} \hat{n} \cdot \vec{S}_1 \hat{n} \cdot \vec{v}_1 \vec{S}_1 \cdot \vec{v}_1 + \\ & 3 \hat{n} \cdot \vec{S}_1 \hat{n} \cdot \vec{v}_2 \vec{S}_1 \cdot \vec{v}_1 + 3 \hat{n} \cdot \vec{S}_1 \hat{n} \cdot \vec{v}_1 \vec{S}_1 \cdot \vec{v}_2 - \frac{7}{3} \hat{n} \cdot \vec{S}_1 \hat{n} \cdot \vec{v}_2 \vec{S}_1 \cdot \vec{v}_2 - \frac{1}{6} \left( \hat{n} \cdot \vec{S}_1 \right)^2 \vec{a}_1 \cdot \vec{a}_1 - \frac{1}{3} \left( \hat{n} \cdot \vec{S}_1 \right)^2 \vec{a}_1 \cdot \vec{a}_2 - \\ & \frac{2}{3} \hat{n} \cdot \vec{S}_1 \hat{n} \cdot \vec{S}_1 \vec{a}_1 \cdot \vec{v}_2 + \frac{16}{3} \hat{n} \cdot \vec{a}_1 \hat{n} \cdot \vec{v}_1 \vec{S}_1 \cdot \vec{S}_1 - \frac{5}{3} \hat{n} \cdot \vec{a}_2 \hat{n} \cdot \vec{v}_1 \vec{S}_1 \cdot \vec{S}_1 - \frac{5}{3} \hat{n} \cdot \vec{a}_1 \hat{n} \cdot \vec{v}_2 \vec{S}_1 \cdot \vec{S}_1 + \\ & \frac{5}{6} \vec{a}_1 \cdot \vec{v}_2 \vec{S}_1 \cdot \vec{S}_1 - \frac{10}{3} \left( \hat{n} \cdot \vec{v}_1 \right)^2 \vec{S}_1 \cdot \vec{S}_1 - \frac{2}{3} \left( \hat{n} \cdot \vec{v}_2 \right)^2 \vec{S}_1 \cdot \vec{S}_1 + 3 \hat{n} \cdot \vec{v}_1 \hat{n} \cdot \vec{v}_2 \vec{S}_1 \cdot \vec{S}_1 - \frac{2}{3} \hat{n} \cdot \vec{a}_1 \hat{n} \cdot \vec{S}_1 \vec{S}_1 \cdot \vec{a}_1 + \\ & \frac{5}{6} \hat{n} \cdot \vec{a}_2 \hat{n} \cdot \vec{S}_1 \vec{S}_1 \cdot \vec{a}_1 + \frac{5}{6} \hat{n} \cdot \vec{S}_1 \hat{n} \cdot \vec{v}_1 \vec{S}_1 \cdot \vec{a}_1 - \frac{2}{3} \hat{n} \cdot \vec{S}_1 \hat{n} \cdot \vec{v}_2 \vec{S}_1 \cdot \vec{a}_1 - \frac{1}{6} \vec{S}_1 \cdot \vec{v}_1 \vec{S}_1 \cdot \vec{a}_1 + \\ & \frac{1}{3} \vec{S}_1 \cdot \vec{v}_2 \vec{S}_1 \cdot \vec{a}_1 - \frac{2}{3} \hat{n} \cdot \vec{a}_1 \hat{n} \cdot \vec{S}_1 \vec{S}_1 \cdot \vec{a}_2 - \frac{2}{3} \hat{n} \cdot \vec{S}_1 \hat{n} \cdot \vec{v}_1 \vec{S}_1 \cdot \vec{a}_2 + \frac{1}{3} \vec{S}_1 \cdot \vec{v}_1 \vec{S}_1 \cdot \vec{a}_2 - \frac{5}{12} \vec{S}_1 \cdot \vec{a}_1 \vec{S}_1 \cdot \vec{a}_2 + \\ & \frac{4}{3} \left( \hat{n} \cdot \vec{a}_1 \right)^2 \vec{S}_1 \cdot \vec{S}_1 - \frac{5}{6} \hat{n} \cdot \vec{a}_1 \hat{n} \cdot \vec{a}_2 \vec{S}_1 \cdot \vec{S}_1 - \frac{5}{12} \vec{a}_1 \cdot \vec{a}_1 \vec{S}_1 \cdot \vec{S}_1 + \frac{5}{12} \vec{a}_1 \cdot \vec{a}_2 \vec{S}_1 \cdot \vec{S}_1 - \frac{13}{6} \hat{n} \cdot \vec{S}_1 \hat{n} \cdot \vec{a}_1 \vec{S}_1 \cdot \vec{v}_1 + \\ & \frac{7}{3} \hat{n} \cdot \vec{S}_1 \hat{n} \cdot \vec{a}_2 \vec{S}_1 \cdot \vec{v}_1 - \frac{1}{6} \hat{n} \cdot \vec{S}_1 \hat{n} \cdot \vec{v}_1 \vec{S}_1 \cdot \vec{v}_1 + \frac{17}{6} \vec{S}_1 \cdot \vec{a}_1 \vec{S}_1 \cdot \vec{v}_1 - \frac{7}{6} \vec{S}_1 \cdot \vec{a}_2 \vec{S}_1 \cdot \vec{v}_1 - \frac{1}{6} \vec{S}_1 \cdot \vec{v}_1 \vec{S}_1 \cdot \vec{v}_1 - \\ & \frac{2}{3} \hat{n} \cdot \vec{S}_1 \hat{n} \cdot \vec{a}_1 \vec{S}_1 \cdot \vec{v}_2 + 3 \hat{n} \cdot \vec{S}_1 \hat{n} \cdot \vec{v}_1 \vec{S}_1 \cdot \vec{v}_2 - \frac{7}{3} \hat{n} \cdot \vec{S}_1 \hat{n} \cdot \vec{v}_2 \vec{S}_1 \cdot \vec{v}_2 - \frac{7}{6} \vec{S}_1 \cdot \vec{a}_1 \vec{S}_1 \cdot \vec{v}_2 - \frac{3}{2} \vec{S}_1 \cdot \vec{v}_1 \vec{S}_1 \cdot \vec{v}_2 + \end{aligned}$$



$$\begin{aligned}
& \frac{10}{3} \hat{n} \cdot \vec{v}_2 \vec{S}_1 \cdot \vec{S}_1 \vec{v}_1 \cdot \vec{v}_1 - \frac{1}{3} \hat{n} \cdot \vec{S}_1 \vec{S}_1 \cdot \vec{a}_1 \vec{v}_1 \cdot \vec{v}_1 - \hat{n} \cdot \vec{S}_1 \vec{S}_1 \cdot \vec{a}_2 \vec{v}_1 \cdot \vec{v}_1 + \frac{11}{6} \hat{n} \cdot \vec{a}_1 \vec{S}_1 \cdot \vec{S}_1 \vec{v}_1 \cdot \vec{v}_1 - \\
& \hat{n} \cdot \vec{S}_1 \vec{S}_1 \cdot \vec{v}_1 \vec{v}_1 \cdot \vec{v}_1 - \frac{1}{3} \hat{n} \cdot \vec{S}_1 \vec{S}_1 \cdot \vec{v}_2 \vec{v}_1 \cdot \vec{v}_1 + \frac{13}{6} \hat{n} \cdot \vec{a}_1 \left( \hat{n} \cdot \vec{S}_1 \right)^2 \vec{v}_1 \cdot \vec{v}_2 - \frac{16}{3} \hat{n} \cdot \vec{S}_1 \hat{n} \cdot \vec{S}_1 \hat{n} \cdot \vec{v}_2 \vec{v}_1 \cdot \vec{v}_2 - \\
& \frac{13}{6} \hat{n} \cdot \vec{S}_1 \vec{S}_1 \cdot \vec{v}_1 \vec{v}_1 \cdot \vec{v}_2 + \frac{4}{3} \hat{n} \cdot \vec{S}_1 \vec{S}_1 \cdot \vec{v}_2 \vec{v}_1 \cdot \vec{v}_2 + \frac{10}{3} \hat{n} \cdot \vec{v}_2 \vec{S}_1 \cdot \vec{S}_1 \vec{v}_1 \cdot \vec{v}_2 + \frac{13}{6} \hat{n} \cdot \vec{S}_1 \vec{S}_1 \cdot \vec{a}_1 \vec{v}_1 \cdot \vec{v}_2 - \\
& \frac{8}{3} \hat{n} \cdot \vec{a}_1 \vec{S}_1 \cdot \vec{S}_1 \vec{v}_1 \cdot \vec{v}_2 + \frac{23}{6} \hat{n} \cdot \vec{S}_1 \vec{S}_1 \cdot \vec{v}_1 \vec{v}_1 \cdot \vec{v}_2 + \frac{4}{3} \hat{n} \cdot \vec{S}_1 \vec{S}_1 \cdot \vec{v}_2 \vec{v}_1 \cdot \vec{v}_2 - \frac{4}{3} \hat{n} \cdot \vec{a}_1 \left( \hat{n} \cdot \vec{S}_1 \right)^2 \vec{v}_2 \cdot \vec{v}_2 + \\
& \frac{2}{3} \hat{n} \cdot \vec{S}_1 \vec{S}_1 \cdot \vec{v}_1 \vec{v}_2 \cdot \vec{v}_2 - \frac{5}{6} \hat{n} \cdot \vec{S}_1 \vec{S}_1 \cdot \vec{a}_1 \vec{v}_2 \cdot \vec{v}_2 + \frac{5}{6} \hat{n} \cdot \vec{a}_1 \vec{S}_1 \cdot \vec{S}_1 \vec{v}_2 \cdot \vec{v}_2 - \frac{7}{3} \hat{n} \cdot \vec{S}_1 \vec{S}_1 \cdot \vec{v}_1 \vec{v}_2 \cdot \vec{v}_2 \Big) + \frac{1}{r^4} \\
& \left( -\frac{19}{4} \left( \hat{n} \cdot \vec{S}_1 \right)^2 \left( \hat{n} \cdot \vec{v}_1 \right)^4 - \frac{41}{8} \vec{S}_1 \cdot \vec{S}_1 \left( \hat{n} \cdot \vec{v}_1 \right)^4 + 14 \left( \hat{n} \cdot \vec{S}_1 \right)^2 \hat{n} \cdot \vec{v}_2 \left( \hat{n} \cdot \vec{v}_1 \right)^3 + \frac{25}{2} \hat{n} \cdot \vec{v}_2 \vec{S}_1 \cdot \vec{S}_1 \left( \hat{n} \cdot \vec{v}_1 \right)^3 + \right. \\
& \frac{17}{2} \hat{n} \cdot \vec{S}_1 \vec{S}_1 \cdot \vec{v}_1 \left( \hat{n} \cdot \vec{v}_1 \right)^3 - \frac{7}{2} \hat{n} \cdot \vec{S}_1 \vec{S}_1 \cdot \vec{v}_2 \left( \hat{n} \cdot \vec{v}_1 \right)^3 - \frac{27}{4} \left( \hat{n} \times \vec{S}_1 \cdot \vec{v}_1 \right)^2 \left( \hat{n} \cdot \vec{v}_1 \right)^2 - \\
& 12 \left( \hat{n} \cdot \vec{S}_1 \right)^2 \left( \hat{n} \cdot \vec{v}_2 \right)^2 \left( \hat{n} \cdot \vec{v}_1 \right)^2 - \frac{15}{4} \left( \vec{S}_1 \cdot \vec{v}_1 \right)^2 \left( \hat{n} \cdot \vec{v}_1 \right)^2 - \frac{1}{2} \left( \vec{S}_1 \cdot \vec{v}_2 \right)^2 \left( \hat{n} \cdot \vec{v}_1 \right)^2 - \\
& 12 \left( \hat{n} \cdot \vec{v}_2 \right)^2 \vec{S}_1 \cdot \vec{S}_1 \left( \hat{n} \cdot \vec{v}_1 \right)^2 - 18 \hat{n} \cdot \vec{S}_1 \hat{n} \cdot \vec{v}_2 \vec{S}_1 \cdot \vec{v}_1 \left( \hat{n} \cdot \vec{v}_1 \right)^2 + 6 \hat{n} \cdot \vec{S}_1 \hat{n} \cdot \vec{v}_2 \vec{S}_1 \cdot \vec{v}_2 \left( \hat{n} \cdot \vec{v}_1 \right)^2 + \\
& 3 \vec{S}_1 \cdot \vec{v}_1 \vec{S}_1 \cdot \vec{v}_2 \left( \hat{n} \cdot \vec{v}_1 \right)^2 + 9 \left( \hat{n} \cdot \vec{S}_1 \right)^2 \vec{v}_1 \cdot \vec{v}_1 \left( \hat{n} \cdot \vec{v}_1 \right)^2 + 2 \vec{S}_1 \cdot \vec{S}_1 \vec{v}_1 \cdot \vec{v}_1 \left( \hat{n} \cdot \vec{v}_1 \right)^2 - \\
& \frac{21}{4} \left( \hat{n} \cdot \vec{S}_1 \right)^2 \vec{v}_1 \cdot \vec{v}_2 \left( \hat{n} \cdot \vec{v}_1 \right)^2 - \frac{25}{4} \vec{S}_1 \cdot \vec{S}_1 \vec{v}_1 \cdot \vec{v}_2 \left( \hat{n} \cdot \vec{v}_1 \right)^2 + \frac{3}{2} \left( \hat{n} \cdot \vec{S}_1 \right)^2 \vec{v}_2 \cdot \vec{v}_2 \left( \hat{n} \cdot \vec{v}_1 \right)^2 + \\
& 2 \vec{S}_1 \cdot \vec{S}_1 \vec{v}_2 \cdot \vec{v}_2 \left( \hat{n} \cdot \vec{v}_1 \right)^2 + 6 \hat{n} \cdot \vec{v}_2 \left( \vec{S}_1 \cdot \vec{v}_1 \right)^2 \hat{n} \cdot \vec{v}_1 - 6 \hat{n} \times \vec{S}_1 \cdot \vec{v}_1 \vec{S}_1 \times \vec{v}_1 \cdot \vec{v}_2 \hat{n} \cdot \vec{v}_1 + \\
& 18 \left( \hat{n} \times \vec{S}_1 \cdot \vec{v}_1 \right)^2 \hat{n} \cdot \vec{v}_2 \hat{n} \cdot \vec{v}_1 + 12 \hat{n} \cdot \vec{S}_1 \left( \hat{n} \cdot \vec{v}_2 \right)^2 \vec{S}_1 \cdot \vec{v}_1 \hat{n} \cdot \vec{v}_1 - 4 \hat{n} \cdot \vec{v}_2 \vec{S}_1 \cdot \vec{v}_1 \vec{S}_1 \cdot \vec{v}_2 \hat{n} \cdot \vec{v}_1 - \\
& \frac{39}{2} \left( \hat{n} \cdot \vec{S}_1 \right)^2 \hat{n} \cdot \vec{v}_2 \vec{v}_1 \cdot \vec{v}_1 \hat{n} \cdot \vec{v}_1 - 3 \hat{n} \cdot \vec{v}_2 \vec{S}_1 \cdot \vec{S}_1 \vec{v}_1 \cdot \vec{v}_1 \hat{n} \cdot \vec{v}_1 - \frac{9}{2} \hat{n} \cdot \vec{S}_1 \vec{S}_1 \cdot \vec{v}_1 \vec{v}_1 \cdot \vec{v}_1 \hat{n} \cdot \vec{v}_1 + \\
& \frac{13}{2} \hat{n} \cdot \vec{S}_1 \vec{S}_1 \cdot \vec{v}_2 \vec{v}_1 \cdot \vec{v}_1 \hat{n} \cdot \vec{v}_1 + 6 \left( \hat{n} \cdot \vec{S}_1 \right)^2 \hat{n} \cdot \vec{v}_2 \vec{v}_1 \cdot \vec{v}_2 \hat{n} \cdot \vec{v}_1 + 8 \hat{n} \cdot \vec{v}_2 \vec{S}_1 \cdot \vec{S}_1 \vec{v}_1 \cdot \vec{v}_2 \hat{n} \cdot \vec{v}_1 + \\
& 6 \hat{n} \cdot \vec{S}_1 \vec{S}_1 \cdot \vec{v}_1 \vec{v}_1 \cdot \vec{v}_2 \hat{n} \cdot \vec{v}_1 - 2 \hat{n} \cdot \vec{S}_1 \vec{S}_1 \cdot \vec{v}_2 \vec{v}_1 \cdot \vec{v}_2 \hat{n} \cdot \vec{v}_1 - 2 \hat{n} \cdot \vec{S}_1 \vec{S}_1 \cdot \vec{v}_1 \vec{v}_2 \cdot \vec{v}_2 \hat{n} \cdot \vec{v}_1 - \frac{3}{2} \left( \vec{S}_1 \times \vec{v}_1 \cdot \vec{v}_2 \right)^2 - \\
& 18 \left( \hat{n} \times \vec{S}_1 \cdot \vec{v}_1 \right)^2 \left( \hat{n} \cdot \vec{v}_2 \right)^2 - 2 \left( \hat{n} \cdot \vec{v}_2 \right)^2 \left( \vec{S}_1 \cdot \vec{v}_1 \right)^2 - \frac{5}{4} \left( \hat{n} \cdot \vec{S}_1 \right)^2 \left( \vec{v}_1 \cdot \vec{v}_1 \right)^2 + \frac{9}{8} \vec{S}_1 \cdot \vec{S}_1 \left( \vec{v}_1 \cdot \vec{v}_1 \right)^2 - \\
& \frac{1}{2} \left( \hat{n} \cdot \vec{S}_1 \right)^2 \left( \vec{v}_1 \cdot \vec{v}_2 \right)^2 - \vec{S}_1 \cdot \vec{S}_1 \left( \vec{v}_1 \cdot \vec{v}_2 \right)^2 + 12 \hat{n} \times \vec{S}_1 \cdot \vec{v}_1 \vec{S}_1 \times \vec{v}_1 \cdot \vec{v}_2 \hat{n} \cdot \vec{v}_2 - \frac{3}{4} \left( \hat{n} \times \vec{S}_1 \cdot \vec{v}_1 \right)^2 \vec{v}_1 \cdot \vec{v}_1 + \\
& 12 \left( \hat{n} \cdot \vec{S}_1 \right)^2 \left( \hat{n} \cdot \vec{v}_2 \right)^2 \vec{v}_1 \cdot \vec{v}_1 - \frac{1}{4} \left( \vec{S}_1 \cdot \vec{v}_1 \right)^2 \vec{v}_1 \cdot \vec{v}_1 + \left( \vec{S}_1 \cdot \vec{v}_2 \right)^2 \vec{v}_1 \cdot \vec{v}_1 + 4 \hat{n} \cdot \vec{S}_1 \hat{n} \cdot \vec{v}_2 \vec{S}_1 \cdot \vec{v}_1 \vec{v}_1 \cdot \vec{v}_1 - \\
& 8 \hat{n} \cdot \vec{S}_1 \hat{n} \cdot \vec{v}_2 \vec{S}_1 \cdot \vec{v}_2 \vec{v}_1 \cdot \vec{v}_1 - \vec{S}_1 \cdot \vec{v}_1 \vec{S}_1 \cdot \vec{v}_2 \vec{v}_1 \cdot \vec{v}_1 - 3 \left( \hat{n} \times \vec{S}_1 \cdot \vec{v}_1 \right)^2 \vec{v}_1 \cdot \vec{v}_2 - \frac{3}{2} \left( \vec{S}_1 \cdot \vec{v}_1 \right)^2 \vec{v}_1 \cdot \vec{v}_2 - \\
& 4 \hat{n} \cdot \vec{S}_1 \hat{n} \cdot \vec{v}_2 \vec{S}_1 \cdot \vec{v}_1 \vec{v}_1 \cdot \vec{v}_2 + \vec{S}_1 \cdot \vec{v}_1 \vec{S}_1 \cdot \vec{v}_2 \vec{v}_1 \cdot \vec{v}_2 + \frac{13}{4} \left( \hat{n} \cdot \vec{S}_1 \right)^2 \vec{v}_1 \cdot \vec{v}_1 \vec{v}_1 \cdot \vec{v}_2 + \frac{3}{4} \vec{S}_1 \cdot \vec{S}_1 \vec{v}_1 \cdot \vec{v}_1 \vec{v}_1 \cdot \vec{v}_2 + \\
& \left. 3 \left( \hat{n} \times \vec{S}_1 \cdot \vec{v}_1 \right)^2 \vec{v}_2 \cdot \vec{v}_2 + \frac{1}{2} \left( \vec{S}_1 \cdot \vec{v}_1 \right)^2 \vec{v}_2 \cdot \vec{v}_2 - 2 \left( \hat{n} \cdot \vec{S}_1 \right)^2 \vec{v}_1 \cdot \vec{v}_1 \vec{v}_2 \cdot \vec{v}_2 \right) + \frac{1}{3} \frac{2}{\vec{S}_1 \cdot \vec{S}_1} \log \left( \frac{r}{R_\theta} \right) - \frac{\vec{S}_1 \cdot \vec{S}_1}{6 \epsilon_d} \Big\}
\end{aligned}$$

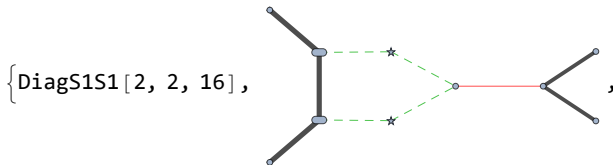

$$\begin{aligned}
G^2 m_2 \Bigg( & -\frac{1}{4} \left( \hat{n} \cdot \vec{S}_1 \right)^2 - \frac{1}{4} \frac{2}{\vec{S}_1 \cdot \vec{S}_1} + \frac{1}{r} \left( -\frac{1}{2} \hat{n} \cdot \vec{a}_2 \left( \hat{n} \cdot \vec{S}_1 \right)^2 + \hat{n} \cdot \vec{S}_1 \hat{n} \cdot \vec{v}_1 \hat{n} \cdot \vec{S}_1 - \hat{n} \cdot \vec{S}_1 \hat{n} \cdot \vec{v}_2 \hat{n} \cdot \vec{S}_1 + \right. \\
& \frac{1}{2} \frac{1}{\vec{S}_1 \cdot \vec{a}_2} \hat{n} \cdot \vec{S}_1 + \frac{1}{2} \frac{2}{\vec{S}_1 \cdot \vec{v}_2} \hat{n} \cdot \vec{S}_1 + \frac{1}{2} \hat{n} \cdot \vec{S}_1 \hat{n} \cdot \vec{a}_1 \hat{n} \cdot \vec{S}_1 - \hat{n} \cdot \vec{a}_2 \vec{S}_1 \cdot \vec{S}_1 + 2 \hat{n} \cdot \vec{v}_1 \vec{S}_1 \cdot \vec{S}_1 -
\end{aligned}$$

[illegible]

$$\begin{aligned}
& \frac{1}{2} \hat{n} \cdot \vec{a}_1 \left( \hat{n} \cdot \vec{S}_1 \right)^2 \vec{v}_1 \cdot \vec{v}_1 + 2 \hat{n} \cdot \vec{S}_1 \hat{n} \cdot \vec{S}_1 \hat{n} \cdot \vec{v}_2 \vec{v}_1 \cdot \vec{v}_1 - \hat{n} \cdot \vec{S}_1 \vec{S}_1 \cdot \vec{v}_1 \vec{v}_1 \cdot \vec{v}_1 - \frac{1}{2} \hat{n} \cdot \vec{S}_1 \vec{S}_1 \cdot \vec{v}_2 \vec{v}_1 \cdot \vec{v}_1 + \\
& 3 \hat{n} \cdot \vec{v}_2 \vec{S}_1 \cdot \vec{S}_1 \vec{v}_1 \cdot \vec{v}_1 + \frac{1}{2} \hat{n} \cdot \vec{a}_1 \vec{S}_1 \cdot \vec{S}_1 \vec{v}_1 \cdot \vec{v}_1 + \frac{1}{2} \hat{n} \cdot \vec{a}_2 \vec{S}_1 \cdot \vec{S}_1 \vec{v}_1 \cdot \vec{v}_1 + \hat{n} \cdot \vec{S}_1 \vec{S}_1 \cdot \vec{v}_1 \vec{v}_1 \cdot \vec{v}_1 - \\
& \frac{1}{2} \hat{n} \cdot \vec{S}_1 \vec{S}_1 \cdot \vec{v}_2 \vec{v}_1 \cdot \vec{v}_1 + \frac{1}{2} \hat{n} \cdot \vec{a}_1 \left( \hat{n} \cdot \vec{S}_1 \right)^2 \vec{v}_1 \cdot \vec{v}_2 - 4 \hat{n} \cdot \vec{S}_1 \hat{n} \cdot \vec{S}_1 \hat{n} \cdot \vec{v}_2 \vec{v}_1 \cdot \vec{v}_2 - \frac{1}{2} \hat{n} \cdot \vec{S}_1 \vec{S}_1 \cdot \vec{v}_1 \vec{v}_1 \cdot \vec{v}_2 + \\
& \hat{n} \cdot \vec{S}_1 \vec{S}_1 \cdot \vec{v}_2 \vec{v}_1 \cdot \vec{v}_2 - 4 \hat{n} \cdot \vec{v}_2 \vec{S}_1 \cdot \vec{S}_1 \vec{v}_1 \cdot \vec{v}_2 - \frac{3}{2} \hat{n} \cdot \vec{S}_1 \vec{S}_1 \cdot \vec{v}_1 \vec{v}_1 \cdot \vec{v}_2 + \hat{n} \cdot \vec{S}_1 \vec{S}_1 \cdot \vec{v}_2 \vec{v}_1 \cdot \vec{v}_2 + \hat{n} \cdot \vec{S}_1 \vec{S}_1 \cdot \vec{v}_1 \vec{v}_2 \cdot \vec{v}_2 \Big) + \\
& \frac{1}{r^4} \left( -\frac{9}{4} \left( \hat{n} \cdot \vec{S}_1 \right)^2 \left( \hat{n} \cdot \vec{v}_1 \right)^4 - \frac{3}{8} \vec{S}_1 \cdot \vec{S}_1 \left( \hat{n} \cdot \vec{v}_1 \right)^4 + 12 \left( \hat{n} \cdot \vec{S}_1 \right)^2 \hat{n} \cdot \vec{v}_2 \left( \hat{n} \cdot \vec{v}_1 \right)^3 + \frac{3}{2} \hat{n} \cdot \vec{S}_1 \vec{S}_1 \cdot \vec{v}_1 \left( \hat{n} \cdot \vec{v}_1 \right)^3 - \right. \\
& 3 \hat{n} \cdot \vec{S}_1 \vec{S}_1 \cdot \vec{v}_2 \left( \hat{n} \cdot \vec{v}_1 \right)^3 + \frac{3}{4} \left( \hat{n} \times \vec{S}_1 \cdot \vec{v}_1 \right)^2 \left( \hat{n} \cdot \vec{v}_1 \right)^2 - 12 \left( \hat{n} \cdot \vec{S}_1 \right)^2 \left( \hat{n} \cdot \vec{v}_2 \right)^2 \left( \hat{n} \cdot \vec{v}_1 \right)^2 - \\
& \frac{1}{4} \left( \vec{S}_1 \cdot \vec{v}_1 \right)^2 \left( \hat{n} \cdot \vec{v}_1 \right)^2 - \frac{1}{2} \left( \vec{S}_1 \cdot \vec{v}_2 \right)^2 \left( \hat{n} \cdot \vec{v}_1 \right)^2 - 3 \hat{n} \cdot \vec{S}_1 \hat{n} \cdot \vec{v}_2 \vec{S}_1 \cdot \vec{v}_1 \left( \hat{n} \cdot \vec{v}_1 \right)^2 + \\
& 6 \hat{n} \cdot \vec{S}_1 \hat{n} \cdot \vec{v}_2 \vec{S}_1 \cdot \vec{v}_2 \left( \hat{n} \cdot \vec{v}_1 \right)^2 + \frac{1}{2} \vec{S}_1 \cdot \vec{v}_1 \vec{S}_1 \cdot \vec{v}_2 \left( \hat{n} \cdot \vec{v}_1 \right)^2 + \frac{3}{2} \left( \hat{n} \cdot \vec{S}_1 \right)^2 \vec{v}_1 \cdot \vec{v}_1 \left( \hat{n} \cdot \vec{v}_1 \right)^2 - \\
& \frac{1}{2} \vec{S}_1 \cdot \vec{S}_1 \vec{v}_1 \cdot \vec{v}_1 \left( \hat{n} \cdot \vec{v}_1 \right)^2 - \frac{9}{2} \left( \hat{n} \cdot \vec{S}_1 \right)^2 \vec{v}_1 \cdot \vec{v}_2 \left( \hat{n} \cdot \vec{v}_1 \right)^2 + \frac{3}{2} \left( \hat{n} \cdot \vec{S}_1 \right)^2 \vec{v}_2 \cdot \vec{v}_2 \left( \hat{n} \cdot \vec{v}_1 \right)^2 + \\
& 2 \hat{n} \times \vec{S}_1 \cdot \vec{v}_1 \vec{S}_1 \times \vec{v}_1 \cdot \vec{v}_2 \hat{n} \cdot \vec{v}_1 - 6 \left( \hat{n} \times \vec{S}_1 \cdot \vec{v}_1 \right)^2 \hat{n} \cdot \vec{v}_2 \hat{n} \cdot \vec{v}_1 - 3 \left( \hat{n} \cdot \vec{S}_1 \right)^2 \hat{n} \cdot \vec{v}_2 \vec{v}_1 \cdot \vec{v}_1 \hat{n} \cdot \vec{v}_1 - \\
& 2 \hat{n} \cdot \vec{v}_2 \vec{S}_1 \cdot \vec{S}_1 \vec{v}_1 \cdot \vec{v}_1 \hat{n} \cdot \vec{v}_1 + \frac{1}{2} \hat{n} \cdot \vec{S}_1 \vec{S}_1 \cdot \vec{v}_1 \vec{v}_1 \cdot \vec{v}_1 \hat{n} \cdot \vec{v}_1 + \hat{n} \cdot \vec{S}_1 \vec{S}_1 \cdot \vec{v}_2 \vec{v}_1 \cdot \vec{v}_1 \hat{n} \cdot \vec{v}_1 + \\
& 6 \left( \hat{n} \cdot \vec{S}_1 \right)^2 \hat{n} \cdot \vec{v}_2 \vec{v}_1 \cdot \vec{v}_2 \hat{n} \cdot \vec{v}_1 + \hat{n} \cdot \vec{S}_1 \vec{S}_1 \cdot \vec{v}_1 \vec{v}_1 \cdot \vec{v}_2 \hat{n} \cdot \vec{v}_1 - 2 \hat{n} \cdot \vec{S}_1 \vec{S}_1 \cdot \vec{v}_2 \vec{v}_1 \cdot \vec{v}_2 \hat{n} \cdot \vec{v}_1 + \\
& \frac{1}{2} \left( \vec{S}_1 \times \vec{v}_1 \cdot \vec{v}_2 \right)^2 + 6 \left( \hat{n} \times \vec{S}_1 \cdot \vec{v}_1 \right)^2 \left( \hat{n} \cdot \vec{v}_2 \right)^2 - \frac{1}{4} \left( \hat{n} \cdot \vec{S}_1 \right)^2 \left( \vec{v}_1 \cdot \vec{v}_1 \right)^2 + \frac{7}{8} \vec{S}_1 \cdot \vec{S}_1 \left( \vec{v}_1 \cdot \vec{v}_1 \right)^2 - \\
& \frac{1}{2} \left( \hat{n} \cdot \vec{S}_1 \right)^2 \left( \vec{v}_1 \cdot \vec{v}_2 \right)^2 - 4 \hat{n} \times \vec{S}_1 \cdot \vec{v}_1 \vec{S}_1 \times \vec{v}_1 \cdot \vec{v}_2 \hat{n} \cdot \vec{v}_2 - \frac{5}{4} \left( \hat{n} \times \vec{S}_1 \cdot \vec{v}_1 \right)^2 \vec{v}_1 \cdot \vec{v}_1 - \\
& \frac{3}{4} \left( \vec{S}_1 \cdot \vec{v}_1 \right)^2 \vec{v}_1 \cdot \vec{v}_1 + 2 \left( \hat{n} \cdot \vec{v}_2 \right)^2 \vec{S}_1 \cdot \vec{S}_1 \vec{v}_1 \cdot \vec{v}_1 + \left( \hat{n} \times \vec{S}_1 \cdot \vec{v}_1 \right)^2 \vec{v}_1 \cdot \vec{v}_2 + \frac{1}{2} \left( \hat{n} \cdot \vec{S}_1 \right)^2 \vec{v}_1 \cdot \vec{v}_1 \vec{v}_1 \cdot \vec{v}_2 + \\
& \left. \frac{1}{2} \vec{S}_1 \cdot \vec{S}_1 \vec{v}_1 \cdot \vec{v}_1 \vec{v}_1 \cdot \vec{v}_2 - \left( \hat{n} \times \vec{S}_1 \cdot \vec{v}_1 \right)^2 \vec{v}_2 \cdot \vec{v}_2 - \frac{1}{2} \vec{S}_1 \cdot \vec{S}_1 \vec{v}_1 \cdot \vec{v}_1 \vec{v}_2 \cdot \vec{v}_2 \right) + \frac{2}{\vec{S}_1 \cdot \vec{S}_1} \log \left( \frac{r}{R_\theta} \right) - \frac{\vec{S}_1 \cdot \vec{S}_1}{2 \epsilon_d} \Big\}
\end{aligned}$$

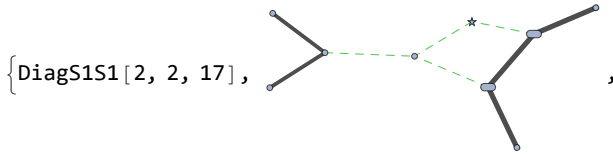

$$\begin{aligned}
& G^2 \left( \frac{1}{r} \left( \frac{1}{6} \hat{n} \cdot \vec{a}_2 \left( \hat{n} \cdot \vec{S}_1 \right)^2 + \frac{2}{3} \hat{n} \cdot \vec{S}_1 \hat{n} \cdot \vec{v}_2 \hat{n} \cdot \vec{S}_1 + \frac{1}{3} \vec{S}_1 \cdot \vec{a}_2 \hat{n} \cdot \vec{S}_1 - \frac{4}{3} \vec{S}_1 \cdot \vec{v}_2 \hat{n} \cdot \vec{S}_1 + \right. \right. \\
& \vec{S}_1 \cdot \vec{a}_2 \hat{n} \cdot \vec{S}_1 + \frac{1}{2} \hat{n} \cdot \vec{S}_1 \hat{n} \cdot \vec{a}_2 \hat{n} \cdot \vec{S}_1 + \hat{n} \cdot \vec{S}_1 \vec{S}_1 \cdot \vec{a}_2 - \frac{5}{6} \hat{n} \cdot \vec{a}_2 \vec{S}_1 \cdot \vec{S}_1 + \frac{2}{3} \hat{n} \cdot \vec{v}_2 \vec{S}_1 \cdot \vec{S}_1 - \\
& \left. \frac{4}{3} \hat{n} \cdot \vec{S}_1 \vec{S}_1 \cdot \vec{v}_2 - \frac{1}{2} \hat{n} \cdot \vec{S}_1 \vec{S}_1 \cdot \vec{a}_2 - 2 \hat{n} \cdot \vec{a}_2 \vec{S}_1 \cdot \vec{S}_1 - \frac{1}{2} \hat{n} \cdot \vec{a}_2 \vec{S}_1 \cdot \vec{S}_1 - \frac{1}{2} \hat{n} \cdot \vec{S}_1 \vec{S}_1 \cdot \vec{a}_2 \right) + \\
& \frac{1}{r^2} \left( \frac{2}{3} \left( \hat{n} \cdot \vec{v}_2 \right)^2 \left( \hat{n} \cdot \vec{S}_1 \right)^2 - \frac{4}{3} \hat{n} \cdot \vec{v}_1 \hat{n} \cdot \vec{v}_2 \left( \hat{n} \cdot \vec{S}_1 \right)^2 - \frac{2}{3} \vec{v}_1 \cdot \vec{v}_2 \left( \hat{n} \cdot \vec{S}_1 \right)^2 - \frac{1}{6} \vec{v}_2 \cdot \vec{v}_2 \left( \hat{n} \cdot \vec{S}_1 \right)^2 - \right. \\
& \frac{4}{3} \hat{n} \cdot \vec{a}_2 \hat{n} \cdot \vec{S}_1 \hat{n} \cdot \vec{v}_1 \hat{n} \cdot \vec{S}_1 - \frac{2}{3} \hat{n} \cdot \vec{a}_1 \hat{n} \cdot \vec{S}_1 \hat{n} \cdot \vec{v}_2 \hat{n} \cdot \vec{S}_1 + \frac{8}{3} \hat{n} \cdot \vec{v}_2 \vec{S}_1 \cdot \vec{v}_1 \hat{n} \cdot \vec{S}_1 + \frac{20}{3} \hat{n} \cdot \vec{v}_1 \vec{S}_1 \cdot \vec{v}_2 \hat{n} \cdot \vec{S}_1 + \\
& \left. \frac{1}{3} \hat{n} \cdot \vec{v}_2 \vec{S}_1 \cdot \vec{v}_2 \hat{n} \cdot \vec{S}_1 - \frac{1}{3} \hat{n} \cdot \vec{S}_1 \vec{a}_1 \cdot \vec{v}_2 \hat{n} \cdot \vec{S}_1 - \frac{1}{3} \hat{n} \cdot \vec{v}_2 \vec{S}_1 \cdot \vec{a}_1 \hat{n} \cdot \vec{S}_1 + \frac{1}{3} \hat{n} \cdot \vec{v}_1 \vec{S}_1 \cdot \vec{a}_2 \hat{n} \cdot \vec{S}_1 + \right. \\
& \left. 4 \hat{n} \cdot \vec{v}_2 \vec{S}_1 \cdot \vec{a}_2 \hat{n} \cdot \vec{S}_1 + \frac{7}{3} \hat{n} \cdot \vec{a}_2 \vec{S}_1 \cdot \vec{v}_1 \hat{n} \cdot \vec{S}_1 + \frac{5}{3} \hat{n} \cdot \vec{a}_1 \vec{S}_1 \cdot \vec{v}_2 \hat{n} \cdot \vec{S}_1 + 2 \hat{n} \cdot \vec{a}_2 \vec{S}_1 \cdot \vec{v}_2 \hat{n} \cdot \vec{S}_1 - \right.
\end{aligned}$$





$\{\text{DiagS1S1}[2, 2, 18],$

[illegible]





$$\begin{aligned} & G^2 \left( \frac{1}{r^2} \left( \hat{n} \cdot \vec{v}_1 \hat{n} \cdot \vec{v}_2 \vec{S}_1 \cdot \vec{S}_1 - \frac{1}{2} \vec{v}_1 \cdot \vec{v}_2 \vec{S}_1 \cdot \vec{S}_1 - \hat{n} \cdot \vec{S}_1 \hat{n} \cdot \vec{v}_2 \vec{S}_1 \cdot \vec{a}_1 + \hat{n} \cdot \vec{a}_2 \hat{n} \cdot \vec{S}_1 \vec{S}_1 \cdot \vec{v}_1 - \hat{n} \cdot \vec{S}_1 \hat{n} \cdot \vec{v}_2 \vec{S}_1 \cdot \vec{v}_1 + \frac{1}{2} \vec{S}_1 \cdot \vec{v}_1 \right. \right. \\ & \quad \frac{1}{\vec{S}_1 \cdot \vec{v}_2} - \hat{n} \cdot \vec{S}_1 \hat{n} \cdot \vec{v}_2 \vec{S}_1 \cdot \vec{a}_1 - 2 \hat{n} \cdot \vec{a}_2 \hat{n} \cdot \vec{v}_1 \vec{S}_1 \cdot \vec{S}_1 + 3 \hat{n} \cdot \vec{a}_1 \hat{n} \cdot \vec{v}_2 \vec{S}_1 \cdot \vec{S}_1 - \frac{3}{2} \vec{a}_1 \cdot \vec{v}_2 \vec{S}_1 \cdot \vec{S}_1 + \hat{n} \cdot \vec{v}_1 \hat{n} \cdot \vec{v}_2 \vec{S}_1 \cdot \vec{S}_1 + \\ & \quad \hat{n} \cdot \vec{a}_2 \hat{n} \cdot \vec{S}_1 \vec{S}_1 \cdot \vec{a}_1 - 2 \hat{n} \cdot \vec{S}_1 \hat{n} \cdot \vec{v}_2 \vec{S}_1 \cdot \vec{a}_1 + \frac{1}{\vec{S}_1 \cdot \vec{v}_2 \vec{S}_1 \cdot \vec{a}_1} - \frac{1}{2} \frac{\vec{S}_1 \cdot \vec{v}_1 \vec{S}_1 \cdot \vec{a}_2}{\vec{S}_1 \cdot \vec{a}_1 \vec{S}_1 \cdot \vec{a}_2} - \hat{n} \cdot \vec{a}_1 \hat{n} \cdot \vec{a}_2 \vec{S}_1 \cdot \vec{S}_1 + \\ & \quad \hat{n} \cdot \frac{1}{\vec{a}_1} \hat{n} \cdot \vec{v}_2 \vec{S}_1 \cdot \vec{S}_1 - \frac{1}{2} \frac{1}{\vec{a}_1 \cdot \vec{v}_2 \vec{S}_1 \cdot \vec{S}_1} + \frac{1}{2} \vec{a}_1 \cdot \vec{a}_2 \vec{S}_1 \cdot \vec{S}_1 + \hat{n} \cdot \frac{1}{\vec{S}_1} \hat{n} \cdot \vec{a}_2 \vec{S}_1 \cdot \vec{v}_1 - \hat{n} \cdot \frac{2}{\vec{S}_1} \hat{n} \cdot \vec{v}_2 \vec{S}_1 \cdot \vec{v}_1 - \\ & \quad \frac{1}{2} \frac{\vec{S}_1 \cdot \vec{a}_2 \vec{S}_1 \cdot \vec{v}_1}{\vec{S}_1 \cdot \vec{v}_2 \vec{S}_1 \cdot \vec{v}_1} + \frac{1}{2} \frac{\vec{S}_1 \cdot \vec{a}_1 \vec{S}_1 \cdot \vec{v}_2}{\vec{S}_1 \cdot \vec{a}_1 \vec{S}_1 \cdot \vec{v}_2} + \frac{1}{2} \vec{S}_1 \cdot \vec{S}_1 \vec{v}_1 \cdot \vec{a}_2 - \frac{1}{2} \vec{S}_1 \cdot \vec{S}_1 \vec{v}_1 \cdot \vec{v}_2 \Big) + \frac{1}{r^3} \\ & \quad \left( -8 \hat{n} \cdot \vec{v}_2 \vec{S}_1 \cdot \vec{S}_1 \left( \hat{n} \cdot \vec{v}_1 \right)^2 + 4 \hat{n} \cdot \vec{a}_2 \vec{S}_1 \cdot \vec{S}_1 \left( \hat{n} \cdot \vec{v}_1 \right)^2 + 2 \hat{n} \cdot \vec{S}_1 \hat{n} \cdot \vec{v}_2 \vec{S}_1 \cdot \vec{v}_1 \hat{n} \cdot \vec{v}_1 - 8 \left( \hat{n} \cdot \vec{v}_2 \right)^2 \vec{S}_1 \cdot \vec{S}_1 \hat{n} \cdot \vec{v}_1 + \right. \\ & \quad 6 \hat{n} \cdot \vec{S}_1 \hat{n} \cdot \vec{v}_2 \vec{S}_1 \cdot \vec{a}_1 \hat{n} \cdot \vec{v}_1 - 8 \hat{n} \cdot \vec{a}_1 \hat{n} \cdot \vec{v}_2 \vec{S}_1 \cdot \vec{S}_1 \hat{n} \cdot \vec{v}_1 + 2 \vec{a}_1 \cdot \vec{v}_2 \vec{S}_1 \cdot \vec{S}_1 \hat{n} \cdot \vec{v}_1 - 4 \hat{n} \cdot \vec{a}_2 \hat{n} \cdot \vec{S}_1 \vec{S}_1 \cdot \vec{v}_1 \hat{n} \cdot \vec{v}_1 + \\ & \quad 6 \hat{n} \cdot \frac{1}{\vec{S}_1} \hat{n} \cdot \vec{v}_2 \vec{S}_1 \cdot \vec{v}_1 \hat{n} \cdot \vec{v}_1 - \frac{3}{2} \frac{1}{\vec{S}_1 \cdot \vec{v}_2 \vec{S}_1 \cdot \vec{v}_1} \hat{n} \cdot \vec{v}_1 + \vec{S}_1 \cdot \vec{a}_2 \vec{S}_1 \cdot \vec{v}_1 \hat{n} \cdot \vec{v}_1 - \frac{1}{2} \frac{1}{\vec{S}_1 \cdot \vec{v}_1 \vec{S}_1 \cdot \vec{v}_2} \hat{n} \cdot \vec{v}_1 - \\ & \quad \frac{3}{2} \vec{S}_1 \cdot \vec{a}_1 \vec{S}_1 \cdot \vec{v}_2 \hat{n} \cdot \vec{v}_1 - 2 \vec{S}_1 \cdot \vec{S}_1 \vec{v}_1 \cdot \vec{a}_2 \hat{n} \cdot \vec{v}_1 + 4 \vec{S}_1 \cdot \frac{1}{\vec{S}_1} \vec{v}_1 \cdot \vec{v}_2 \hat{n} \cdot \vec{v}_1 + 2 \vec{S}_1 \cdot \frac{1}{\vec{S}_1} \vec{v}_2 \cdot \vec{v}_2 \hat{n} \cdot \vec{v}_1 + \\ & \quad \hat{n} \cdot \vec{a}_2 \left( \vec{S}_1 \cdot \vec{v}_1 \right)^2 - \hat{n} \times \vec{S}_1 \cdot \vec{v}_1 \vec{S}_1 \times \vec{v}_1 \cdot \vec{v}_2 - \hat{n} \times \vec{S}_1 \cdot \vec{v}_1 \vec{S}_1 \times \vec{a}_1 \cdot \vec{v}_2 - \hat{n} \times \vec{S}_1 \cdot \vec{v}_1 \vec{S}_1 \times \vec{v}_1 \cdot \vec{v}_2 - \hat{n} \times \vec{S}_1 \cdot \vec{a}_1 \vec{S}_1 \times \vec{v}_1 \cdot \vec{v}_2 + \\ & \quad 4 \hat{n} \times \frac{1}{\vec{S}_1} \cdot \vec{v}_1 \hat{n} \times \vec{S}_1 \cdot \vec{v}_1 \hat{n} \cdot \vec{v}_2 + 4 \hat{n} \times \vec{S}_1 \cdot \vec{a}_1 \hat{n} \times \vec{S}_1 \cdot \vec{v}_1 \hat{n} \cdot \vec{v}_2 + 4 \hat{n} \cdot \vec{S}_1 \left( \hat{n} \cdot \vec{v}_2 \right)^2 \vec{S}_1 \cdot \vec{v}_1 + 4 \hat{n} \cdot \vec{S}_1 \left( \hat{n} \cdot \vec{v}_2 \right)^2 \vec{S}_1 \cdot \vec{a}_1 - \\ & \quad 4 \hat{n} \cdot \vec{a}_1 \left( \hat{n} \cdot \vec{v}_2 \right)^2 \vec{S}_1 \cdot \vec{S}_1 + 2 \hat{n} \cdot \vec{v}_2 \vec{a}_1 \cdot \vec{v}_2 \vec{S}_1 \cdot \vec{S}_1 + 4 \hat{n} \cdot \frac{1}{\vec{S}_1} \left( \hat{n} \cdot \vec{v}_2 \right)^2 \vec{S}_1 \cdot \vec{v}_1 + 2 \hat{n} \cdot \vec{a}_1 \hat{n} \cdot \vec{S}_1 \hat{n} \cdot \vec{v}_2 \vec{S}_1 \cdot \vec{v}_1 - \\ & \quad \hat{n} \cdot \vec{v}_2 \frac{1}{\vec{S}_1} \cdot \vec{v}_1 \vec{S}_1 \cdot \vec{v}_1 - 2 \hat{n} \cdot \vec{v}_2 \vec{S}_1 \cdot \vec{v}_2 \vec{S}_1 \cdot \vec{v}_1 - \frac{1}{2} \hat{n} \cdot \vec{S}_1 \vec{a}_1 \cdot \vec{v}_2 \vec{S}_1 \cdot \vec{v}_1 - \hat{n} \cdot \vec{v}_2 \vec{S}_1 \cdot \vec{a}_1 \vec{S}_1 \cdot \vec{v}_1 - 2 \hat{n} \cdot \vec{v}_2 \frac{1}{\vec{S}_1} \cdot \vec{v}_1 \vec{S}_1 \cdot \vec{v}_2 - \\ & \quad 2 \hat{n} \cdot \vec{v}_2 \vec{S}_1 \cdot \vec{a}_1 \vec{S}_1 \cdot \vec{v}_2 - \frac{1}{2} \hat{n} \cdot \vec{a}_1 \vec{S}_1 \cdot \vec{v}_1 \vec{S}_1 \cdot \vec{v}_2 + \hat{n} \cdot \vec{v}_2 \vec{S}_1 \cdot \vec{S}_1 \vec{v}_1 \cdot \vec{a}_1 + \hat{n} \cdot \vec{S}_1 \vec{S}_1 \cdot \vec{v}_1 \vec{v}_1 \cdot \vec{a}_2 + \hat{n} \cdot \vec{v}_2 \vec{S}_1 \cdot \frac{1}{\vec{S}_1} \vec{v}_1 \cdot \vec{v}_1 - \\ & \quad \hat{n} \cdot \vec{a}_2 \vec{S}_1 \cdot \vec{S}_1 \vec{v}_1 \cdot \vec{v}_1 - \frac{1}{2} \hat{n} \cdot \vec{S}_1 \frac{1}{\vec{S}_1} \cdot \vec{v}_1 \vec{v}_1 \cdot \vec{v}_2 + 4 \hat{n} \cdot \vec{v}_2 \vec{S}_1 \cdot \frac{1}{\vec{S}_1} \vec{v}_1 \cdot \vec{v}_2 - \frac{3}{2} \hat{n} \cdot \vec{S}_1 \vec{S}_1 \cdot \vec{a}_1 \vec{v}_1 \cdot \vec{v}_2 + 2 \hat{n} \cdot \vec{a}_1 \vec{S}_1 \cdot \vec{S}_1 \vec{v}_1 \cdot \vec{v}_2 - \\ & \quad \frac{3}{2} \hat{n} \cdot \frac{1}{\vec{S}_1} \vec{S}_1 \cdot \vec{v}_1 \vec{v}_1 \cdot \vec{v}_2 - \hat{n} \cdot \vec{S}_1 \vec{S}_1 \cdot \vec{v}_1 \vec{v}_2 \cdot \vec{v}_2 - \hat{n} \cdot \vec{S}_1 \vec{S}_1 \cdot \vec{a}_1 \vec{v}_2 \cdot \vec{v}_2 + \hat{n} \cdot \vec{a}_1 \vec{S}_1 \cdot \vec{S}_1 \vec{v}_2 \cdot \vec{v}_2 - \hat{n} \cdot \frac{1}{\vec{S}_1} \vec{S}_1 \cdot \vec{v}_1 \vec{v}_2 \cdot \vec{v}_2 \Big) + \\ & \quad \frac{1}{r^4} \left( 12 \hat{n} \cdot \vec{v}_2 \vec{S}_1 \cdot \vec{S}_1 \left( \hat{n} \cdot \vec{v}_1 \right)^3 + 24 \left( \hat{n} \cdot \vec{v}_2 \right)^2 \vec{S}_1 \cdot \vec{S}_1 \left( \hat{n} \cdot \vec{v}_1 \right)^2 - 12 \hat{n} \cdot \vec{S}_1 \hat{n} \cdot \vec{v}_2 \vec{S}_1 \cdot \vec{v}_1 \left( \hat{n} \cdot \vec{v}_1 \right)^2 + \right. \\ & \quad 2 \vec{S}_1 \cdot \vec{v}_1 \vec{S}_1 \cdot \vec{v}_2 \left( \hat{n} \cdot \vec{v}_1 \right)^2 - 6 \vec{S}_1 \cdot \vec{S}_1 \vec{v}_1 \cdot \vec{v}_2 \left( \hat{n} \cdot \vec{v}_1 \right)^2 - 4 \vec{S}_1 \cdot \vec{S}_1 \vec{v}_2 \cdot \vec{v}_2 \left( \hat{n} \cdot \vec{v}_1 \right)^2 + \\ & \quad 2 \hat{n} \cdot \vec{v}_2 \left( \vec{S}_1 \cdot \vec{v}_1 \right)^2 \hat{n} \cdot \vec{v}_1 + 4 \hat{n} \times \vec{S}_1 \cdot \vec{v}_1 \vec{S}_1 \times \vec{v}_1 \cdot \vec{v}_2 \hat{n} \cdot \vec{v}_1 - 12 \left( \hat{n} \times \vec{S}_1 \cdot \vec{v}_1 \right)^2 \hat{n} \cdot \vec{v}_2 \hat{n} \cdot \vec{v}_1 - \\ & \quad 24 \hat{n} \cdot \vec{S}_1 \left( \hat{n} \cdot \vec{v}_2 \right)^2 \vec{S}_1 \$$

{DiagS1S1[2, 2, 21],

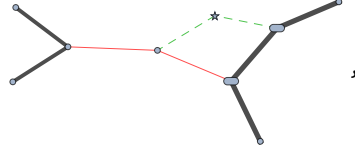

$$\begin{aligned}
 G^2 & \left( \frac{\hat{n} \cdot \vec{S}_1 \vec{S}_1 \cdot \vec{a}_1 - 2 \hat{n} \cdot \vec{a}_1 \vec{S}_1 \cdot \vec{S}_1 - \hat{n} \cdot \vec{v}_1 \vec{S}_1 \cdot \vec{S}_1 + 2 \hat{n} \cdot \vec{S}_1 \vec{S}_1 \cdot \vec{a}_1 + \hat{n} \cdot \vec{S}_1 \vec{S}_1 \cdot \vec{v}_1 - \hat{n} \cdot \vec{a}_1 \vec{S}_1 \cdot \vec{S}_1}{r} + \frac{1}{r^2} \right. \\
 & \left( -3 \left( \hat{n} \times \vec{S}_1 \cdot \vec{v}_1 \right)^2 - 3 \hat{n} \times \vec{S}_1 \cdot \vec{a}_1 \hat{n} \times \vec{S}_1 \cdot \vec{v}_1 + \frac{3}{2} \hat{n} \times \vec{S}_1 \cdot \vec{a}_1 \hat{n} \times \vec{S}_1 \cdot \vec{v}_1 + \frac{3}{2} \hat{n} \times \vec{S}_1 \cdot \vec{v}_1 \hat{n} \times \vec{S}_1 \cdot \vec{v}_1 + \frac{3}{2} \hat{n} \times \vec{S}_1 \cdot \vec{a}_1 \hat{n} \times \vec{S}_1 \cdot \vec{v}_1 + \right. \\
 & 3 \left( \hat{n} \cdot \vec{v}_1 \right)^2 \vec{S}_1 \cdot \vec{S}_1 - 3 \hat{n} \cdot \vec{S}_1 \hat{n} \cdot \vec{v}_1 \vec{S}_1 \cdot \vec{a}_1 - \frac{3}{2} \hat{n} \cdot \vec{a}_1 \hat{n} \cdot \vec{S}_1 \vec{S}_1 \cdot \vec{v}_1 - 2 \hat{n} \cdot \vec{a}_2 \hat{n} \cdot \vec{S}_1 \vec{S}_1 \cdot \vec{v}_1 - 3 \hat{n} \cdot \vec{S}_1 \hat{n} \cdot \vec{v}_1 \vec{S}_1 \cdot \vec{v}_1 - \\
 & \frac{1}{2} \hat{n} \cdot \vec{S}_1 \hat{n} \cdot \vec{v}_1 \vec{S}_1 \cdot \vec{a}_1 + \frac{11}{2} \hat{n} \cdot \vec{a}_1 \hat{n} \cdot \vec{v}_1 \vec{S}_1 \cdot \vec{S}_1 + 2 \hat{n} \cdot \vec{a}_2 \hat{n} \cdot \vec{v}_1 \vec{S}_1 \cdot \vec{S}_1 + \frac{1}{2} \left( \hat{n} \cdot \vec{v}_1 \right)^2 \vec{S}_1 \cdot \vec{S}_1 - \\
 & \hat{n} \cdot \vec{S}_1 \hat{n} \cdot \vec{v}_1 \vec{S}_1 \cdot \vec{a}_1 + 2 \vec{S}_1 \cdot \vec{v}_1 \vec{S}_1 \cdot \vec{a}_1 + \vec{S}_1 \cdot \vec{v}_1 \vec{S}_1 \cdot \vec{a}_2 + \frac{1}{2} \hat{n} \cdot \vec{a}_1 \hat{n} \cdot \vec{v}_1 \vec{S}_1 \cdot \vec{S}_1 - \frac{1}{2} \hat{n} \cdot \vec{S}_1 \hat{n} \cdot \vec{v}_1 \vec{S}_1 \cdot \vec{v}_1 + \\
 & \left. \left. \frac{2}{\vec{S}_1 \cdot \vec{v}_1 \vec{S}_1 \cdot \vec{v}_1} + \vec{S}_1 \cdot \vec{a}_1 \vec{S}_1 \cdot \vec{v}_1 - \vec{S}_1 \cdot \vec{S}_1 \vec{v}_1 \cdot \vec{a}_1 - 2 \vec{S}_1 \cdot \vec{S}_1 \vec{v}_1 \cdot \vec{a}_1 - \vec{S}_1 \cdot \vec{S}_1 \vec{v}_1 \cdot \vec{a}_2 - \vec{S}_1 \cdot \vec{S}_1 \vec{v}_1 \cdot \vec{v}_1 \right) + \frac{1}{r^3} \right. \\
 & \left( -7 \vec{S}_1 \cdot \vec{S}_1 \left( \hat{n} \cdot \vec{v}_1 \right)^3 + 5 \hat{n} \cdot \vec{S}_1 \vec{S}_1 \cdot \vec{v}_1 \left( \hat{n} \cdot \vec{v}_1 \right)^2 + 2 \hat{n} \cdot \vec{S}_1 \vec{S}_1 \cdot \vec{a}_1 \left( \hat{n} \cdot \vec{v}_1 \right)^2 - 3 \hat{n} \cdot \vec{a}_1 \vec{S}_1 \cdot \vec{S}_1 \left( \hat{n} \cdot \vec{v}_1 \right)^2 - \right. \\
 & 2 \hat{n} \cdot \vec{a}_2 \vec{S}_1 \cdot \vec{S}_1 \left( \hat{n} \cdot \vec{v}_1 \right)^2 + 2 \hat{n} \cdot \vec{S}_1 \vec{S}_1 \cdot \vec{v}_1 \left( \hat{n} \cdot \vec{v}_1 \right)^2 + 2 \hat{n} \times \vec{S}_1 \cdot \vec{v}_1 \hat{n} \times \vec{S}_1 \cdot \vec{v}_1 \hat{n} \cdot \vec{v}_1 - 7 \hat{n} \times \vec{S}_1 \cdot \vec{a}_1 \hat{n} \times \vec{S}_1 \cdot \vec{v}_1 \hat{n} \cdot \vec{v}_1 + \\
 & 8 \left( \hat{n} \cdot \vec{v}_2 \right)^2 \vec{S}_1 \cdot \vec{S}_1 \hat{n} \cdot \vec{v}_1 + \hat{n} \cdot \vec{a}_1 \hat{n} \cdot \vec{S}_1 \vec{S}_1 \cdot \vec{v}_1 \hat{n} \cdot \vec{v}_1 + 2 \hat{n} \cdot \vec{a}_2 \hat{n} \cdot \vec{S}_1 \vec{S}_1 \cdot \vec{v}_1 \hat{n} \cdot \vec{v}_1 - 3 \vec{S}_1 \cdot \vec{v}_1 \vec{S}_1 \cdot \vec{v}_1 \hat{n} \cdot \vec{v}_1 - \\
 & 3 \vec{S}_1 \cdot \vec{a}_1 \vec{S}_1 \cdot \vec{v}_1 \hat{n} \cdot \vec{v}_1 - \frac{1}{2} \vec{S}_1 \cdot \vec{a}_2 \vec{S}_1 \cdot \vec{v}_1 \hat{n} \cdot \vec{v}_1 + \frac{7}{2} \vec{S}_1 \cdot \vec{S}_1 \vec{v}_1 \cdot \vec{a}_1 \hat{n} \cdot \vec{v}_1 + \vec{S}_1 \cdot \vec{S}_1 \vec{v}_1 \cdot \vec{a}_2 \hat{n} \cdot \vec{v}_1 + 5 \vec{S}_1 \cdot \vec{S}_1 \vec{v}_1 \cdot \vec{v}_1 \hat{n} \cdot \vec{v}_1 - \\
 & 2 \vec{S}_1 \cdot \vec{S}_1 \vec{v}_2 \cdot \vec{v}_2 \hat{n} \cdot \vec{v}_1 - \frac{3}{2} \hat{n} \cdot \vec{a}_1 \left( \vec{S}_1 \cdot \vec{v}_1 \right)^2 - 2 \hat{n} \cdot \vec{a}_2 \left( \vec{S}_1 \cdot \vec{v}_1 \right)^2 + \frac{3}{2} \hat{n} \times \vec{S}_1 \cdot \vec{v}_1 \vec{S}_1 \times \vec{v}_1 \cdot \vec{a}_1 + 3 \hat{n} \times \vec{S}_1 \cdot \vec{v}_1 \vec{S}_1 \times \vec{v}_1 \cdot \vec{a}_2 - \\
 & 5 \left( \hat{n} \times \vec{S}_1 \cdot \vec{v}_1 \right)^2 \hat{n} \cdot \vec{a}_1 - 6 \left( \hat{n} \times \vec{S}_1 \cdot \vec{v}_1 \right)^2 \hat{n} \cdot \vec{a}_2 - 8 \hat{n} \cdot \vec{S}_1 \left( \hat{n} \cdot \vec{v}_2 \right)^2 \vec{S}_1 \cdot \vec{v}_1 + 4 \hat{n} \cdot \vec{v}_2 \vec{S}_1 \cdot \vec{v}_1 \vec{S}_1 \cdot \vec{v}_2 - \\
 & \frac{1}{2} \hat{n} \cdot \vec{S}_1 \vec{S}_1 \cdot \vec{v}_1 \vec{v}_1 \cdot \vec{a}_1 - \frac{1}{2} \hat{n} \cdot \vec{S}_1 \vec{S}_1 \cdot \vec{v}_1 \vec{v}_1 \cdot \vec{a}_2 - \hat{n} \cdot \vec{S}_1 \vec{S}_1 \cdot \vec{v}_1 \vec{v}_1 \cdot \vec{v}_1 - \hat{n} \cdot \vec{S}_1 \vec{S}_1 \cdot \vec{a}_1 \vec{v}_1 \cdot \vec{v}_1 + \frac{5}{2} \hat{n} \cdot \vec{a}_1 \vec{S}_1 \cdot \vec{S}_1 \vec{v}_1 \cdot \vec{v}_1 + \\
 & 2 \hat{n} \cdot \vec{a}_2 \vec{S}_1 \cdot \vec{S}_1 \vec{v}_1 \cdot \vec{v}_1 - \hat{n} \cdot \vec{S}_1 \vec{S}_1 \cdot \vec{v}_1 \vec{v}_1 \cdot \vec{v}_1 - 4 \hat{n} \cdot \vec{v}_2 \vec{S}_1 \cdot \vec{S}_1 \vec{v}_1 \cdot \vec{v}_2 + 2 \hat{n} \cdot \vec{S}_1 \vec{S}_1 \cdot \vec{v}_1 \vec{v}_2 \cdot \vec{v}_2 \left. \right) + \frac{1}{r^4} \\
 & \left( \frac{15}{4} \vec{S}_1 \cdot \vec{S}_1 \left( \hat{n} \cdot \vec{v}_1 \right)^4 - \frac{15}{4} \hat{n} \cdot \vec{S}_1 \vec{S}_1 \cdot \vec{v}_1 \left( \hat{n} \cdot \vec{v}_1 \right)^3 + \frac{75}{4} \left( \hat{n} \times \vec{S}_1 \cdot \vec{v}_1 \right)^2 \left( \hat{n} \cdot \vec{v}_1 \right)^2 + 5 \left( \vec{S}_1 \cdot \vec{v}_1 \right)^2 \left( \hat{n} \cdot \vec{v}_1 \right)^2 - \right. \\
 & 12 \left( \hat{n} \cdot \vec{v}_2 \right)^2 \vec{S}_1 \cdot \vec{S}_1 \left( \hat{n} \cdot \vec{v}_1 \right)^2 - \frac{31}{4} \vec{S}_1 \cdot \vec{S}_1 \vec{v}_1 \cdot \vec{v}_1 \left( \hat{n} \cdot \vec{v}_1 \right)^2 + 2 \vec{S}_1 \cdot \vec{S}_1 \vec{v}_2 \cdot \vec{v}_2 \left( \hat{n} \cdot \vec{v}_1 \right)^2 + \\
 & 12 \hat{n} \cdot \vec{S}_1 \left( \hat{n} \cdot \vec{v}_2 \right)^2 \vec{S}_1 \cdot \vec{v}_1 \hat{n} \cdot \vec{v}_1 - 4 \hat{n} \cdot \vec{v}_2 \vec{S}_1 \cdot \vec{v}_1 \vec{S}_1 \cdot \vec{v}_2 \hat{n} \cdot \vec{v}_1 + \frac{11}{4} \hat{n} \cdot \vec{S}_1 \vec{S}_1 \cdot \vec{v}_1 \vec{v}_1 \cdot \vec{v}_1 \hat{n} \cdot \vec{v}_1 + \\
 & 8 \hat{n} \cdot \vec{v}_2 \vec{S}_1 \cdot \vec{S}_1 \vec{v}_1 \cdot \vec{v}_2 \hat{n} \cdot \vec{v}_1 - 2 \hat{n} \cdot \vec{S}_1 \vec{S}_1 \cdot \vec{v}_1 \vec{v}_2 \cdot \vec{v}_2 \hat{n} \cdot \vec{v}_1 - 3 \left( \vec{S}_1 \times \vec{v}_1 \cdot \vec{v}_2 \right)^2 - 36 \left( \hat{n} \times \vec{S}_1 \cdot \vec{v}_1 \right)^2 \left( \hat{n} \cdot \vec{v}_2 \right)^2 - \\
 & 8 \left( \hat{n} \cdot \vec{v}_2 \right)^2 \left( \vec{S}_1 \cdot \vec{v}_1 \right)^2 + \vec{S}_1 \cdot \vec{S}_1 \left( \vec{v}_1 \cdot \vec{v}_1 \right)^2 - \vec{S}_1 \cdot \vec{S}_1 \left( \vec{v}_1 \cdot \vec{v}_2 \right)^2 + 24 \hat{n} \times \vec{S}_1 \cdot \vec{v}_1 \vec{S}_1 \times \vec{v}_1 \cdot \vec{v}_2 \hat{n} \cdot \vec{v}_2 - \\
 & \frac{5}{4} \left( \hat{n} \times \vec{S}_1 \cdot \vec{v}_1 \right)^2 \vec{v}_1 \cdot \vec{v}_1 - \left( \vec{S}_1 \cdot \vec{v}_1 \right)^2 \vec{v}_1 \cdot \vec{v}_1 + 8 \left( \hat{n} \cdot \vec{v}_2 \right)^2 \vec{S}_1 \cdot \vec{S}_1 \vec{v}_1 \cdot \vec{v}_1 - 4 \hat{n} \cdot \vec{S}_1 \hat{n} \cdot \vec{v}_2 \vec{S}_1 \cdot \vec{v}_1 \vec{v}_1 \cdot \vec{v}_2 + \\
 & \left. \left. \vec{S}_1 \cdot \vec{v}_1 \vec{S}_1 \cdot \vec{v}_2 \vec{v}_1 \cdot \vec{v}_2 + 6 \left( \hat{n} \times \vec{S}_1 \cdot \vec{v}_1 \right)^2 \vec{v}_2 \cdot \vec{v}_2 + 2 \left( \vec{S}_1 \cdot \vec{v}_1 \right)^2 \vec{v}_2 \cdot \vec{v}_2 - 2 \vec{S}_1 \cdot \vec{S}_1 \vec{v}_1 \cdot \vec{v}_1 \vec{v}_2 \cdot \vec{v}_2 \right) \right) m_2 \}
 \end{aligned}$$

{DiagS1S1[2, 2, 22],

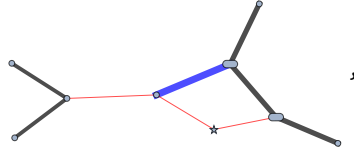

,

$$\begin{aligned}
 G^2 \left( \frac{1}{\rho^2} \left( \frac{1}{2} \left( \hat{n} \times \vec{S}_1 \cdot \vec{v}_1 \right)^2 + \hat{n} \times \vec{S}_1 \cdot \vec{a}_1 \hat{n} \times \vec{S}_1 \cdot \vec{v}_1 + \frac{1}{2} \left( \hat{n} \times \vec{S}_1 \cdot \vec{a}_1 \right)^2 - \left( \vec{S}_1 \cdot \vec{v}_1 \right)^2 - \left( \vec{S}_1 \cdot \vec{a}_1 \right)^2 - \frac{5}{2} \left( \hat{n} \cdot \vec{v}_1 \right)^2 \vec{S}_1 \cdot \vec{S}_1 + \right. \right. \\
 \frac{5}{2} \hat{n} \cdot \vec{S}_1 \hat{n} \cdot \vec{v}_1 \vec{S}_1 \cdot \vec{a}_1 + \frac{5}{2} \hat{n} \cdot \vec{S}_1 \hat{n} \cdot \vec{v}_1 \vec{S}_1 \cdot \vec{v}_1 - 5 \hat{n} \cdot \vec{a}_1 \hat{n} \cdot \vec{v}_1 \vec{S}_1 \cdot \vec{S}_1 + \frac{5}{2} \hat{n} \cdot \vec{a}_1 \hat{n} \cdot \vec{S}_1 \vec{S}_1 \cdot \vec{a}_1 - \frac{5}{2} \left( \hat{n} \cdot \vec{a}_1 \right)^2 \vec{S}_1 \cdot \vec{S}_1 + \\
 \left. \vec{a}_1 \cdot \vec{a}_1 \vec{S}_1 \cdot \vec{S}_1 + \frac{5}{2} \hat{n} \cdot \vec{S}_1 \hat{n} \cdot \vec{a}_1 \vec{S}_1 \cdot \vec{v}_1 - 2 \vec{S}_1 \cdot \vec{a}_1 \vec{S}_1 \cdot \vec{v}_1 + 2 \vec{S}_1 \cdot \vec{S}_1 \vec{v}_1 \cdot \vec{a}_1 + \vec{S}_1 \cdot \vec{S}_1 \vec{v}_1 \cdot \vec{v}_1 \right) + \frac{1}{\rho^3} \\
 \left( 10 \vec{S}_1 \cdot \vec{S}_1 \left( \hat{n} \cdot \vec{v}_1 \right)^3 - 3 \hat{n} \cdot \vec{S}_1 \vec{S}_1 \cdot \vec{v}_1 \left( \hat{n} \cdot \vec{v}_1 \right)^2 - 10 \hat{n} \cdot \vec{v}_2 \vec{S}_1 \cdot \vec{S}_1 \left( \hat{n} \cdot \vec{v}_1 \right)^2 - 7 \hat{n} \cdot \vec{S}_1 \vec{S}_1 \cdot \vec{a}_1 \left( \hat{n} \cdot \vec{v}_1 \right)^2 + \right. \\
 10 \hat{n} \cdot \vec{a}_1 \vec{S}_1 \cdot \vec{S}_1 \left( \hat{n} \cdot \vec{v}_1 \right)^2 - 7 \hat{n} \cdot \vec{S}_1 \vec{S}_1 \cdot \vec{v}_1 \left( \hat{n} \cdot \vec{v}_1 \right)^2 - 2 \hat{n} \times \vec{S}_1 \cdot \vec{v}_1 \hat{n} \times \vec{S}_1 \cdot \vec{v}_1 \hat{n} \cdot \vec{v}_1 + \hat{n} \times \vec{S}_1 \cdot \vec{a}_1 \hat{n} \times \vec{S}_1 \cdot \vec{v}_1 \hat{n} \cdot \vec{v}_1 + \\
 10 \hat{n} \cdot \vec{S}_1 \hat{n} \cdot \vec{v}_2 \vec{S}_1 \cdot \vec{a}_1 \hat{n} \cdot \vec{v}_1 - 10 \hat{n} \cdot \vec{a}_1 \hat{n} \cdot \vec{v}_2 \vec{S}_1 \cdot \vec{S}_1 \hat{n} \cdot \vec{v}_1 + \frac{5}{2} \vec{a}_1 \cdot \vec{v}_2 \vec{S}_1 \cdot \vec{S}_1 \hat{n} \cdot \vec{v}_1 - 3 \hat{n} \cdot \vec{a}_1 \hat{n} \cdot \vec{S}_1 \vec{S}_1 \cdot \vec{v}_1 \hat{n} \cdot \vec{v}_1 + \\
 10 \hat{n} \cdot \vec{S}_1 \hat{n} \cdot \vec{v}_2 \vec{S}_1 \cdot \vec{v}_1 \hat{n} \cdot \vec{v}_1 + \frac{9}{2} \vec{S}_1 \cdot \vec{v}_1 \vec{S}_1 \cdot \vec{v}_1 \hat{n} \cdot \vec{v}_1 - \frac{5}{2} \vec{S}_1 \cdot \vec{v}_2 \vec{S}_1 \cdot \vec{v}_1 \hat{n} \cdot \vec{v}_1 + \frac{9}{2} \vec{S}_1 \cdot \vec{a}_1 \vec{S}_1 \cdot \vec{v}_1 \hat{n} \cdot \vec{v}_1 - \\
 \frac{5}{2} \vec{S}_1 \cdot \vec{a}_1 \vec{S}_1 \cdot \vec{v}_2 \hat{n} \cdot \vec{v}_1 - 5 \vec{S}_1 \cdot \vec{S}_1 \vec{v}_1 \cdot \vec{a}_1 \hat{n} \cdot \vec{v}_1 - 7 \vec{S}_1 \cdot \vec{S}_1 \vec{v}_1 \cdot \vec{v}_1 \hat{n} \cdot \vec{v}_1 + 5 \vec{S}_1 \cdot \vec{S}_1 \vec{v}_1 \cdot \vec{v}_2 \hat{n} \cdot \vec{v}_1 - \\
 \frac{1}{2} \hat{n} \times \vec{S}_1 \cdot \vec{v}_1 \vec{S}_1 \times \vec{v}_1 \cdot \vec{v}_2 - \frac{1}{2} \hat{n} \times \vec{S}_1 \cdot \vec{v}_1 \vec{S}_1 \times \vec{a}_1 \cdot \vec{v}_2 + \hat{n} \times \vec{S}_1 \cdot \vec{v}_1 \vec{S}_1 \times \vec{v}_1 \cdot \vec{a}_1 - \frac{1}{2} \hat{n} \times \vec{S}_1 \cdot \vec{v}_1 \vec{S}_1 \times \vec{v}_1 \cdot \vec{v}_2 - \\
 \frac{1}{2} \hat{n} \times \vec{S}_1 \cdot \vec{a}_1 \vec{S}_1 \times \vec{v}_1 \cdot \vec{v}_2 - 3 \left( \hat{n} \times \vec{S}_1 \cdot \vec{v}_1 \right)^2 \hat{n} \cdot \vec{a}_1 + 2 \hat{n} \times \vec{S}_1 \cdot \vec{v}_1 \hat{n} \times \vec{S}_1 \cdot \vec{v}_1 \hat{n} \cdot \vec{v}_2 + 2 \hat{n} \times \vec{S}_1 \cdot \vec{a}_1 \hat{n} \times \vec{S}_1 \cdot \vec{v}_1 \hat{n} \cdot \vec{v}_2 - \\
 2 \hat{n} \cdot \vec{v}_2 \vec{S}_1 \cdot \vec{v}_1 \vec{S}_1 \cdot \vec{v}_1 - 2 \hat{n} \cdot \vec{v}_2 \vec{S}_1 \cdot \vec{a}_1 \vec{S}_1 \cdot \vec{v}_1 + 2 \hat{n} \cdot \vec{v}_2 \vec{S}_1 \cdot \vec{S}_1 \vec{v}_1 \cdot \vec{a}_1 + \frac{1}{2} \hat{n} \cdot \vec{S}_1 \vec{S}_1 \cdot \vec{v}_1 \vec{v}_1 \cdot \vec{a}_1 + \\
 \frac{1}{2} \hat{n} \cdot \vec{S}_1 \vec{S}_1 \cdot \vec{v}_1 \vec{v}_1 \cdot \vec{v}_1 + 2 \hat{n} \cdot \vec{v}_2 \vec{S}_1 \cdot \vec{S}_1 \vec{v}_1 \cdot \vec{v}_1 + 2 \hat{n} \cdot \vec{S}_1 \vec{S}_1 \cdot \vec{a}_1 \vec{v}_1 \cdot \vec{v}_1 - 2 \hat{n} \cdot \vec{a}_1 \vec{S}_1 \cdot \vec{S}_1 \vec{v}_1 \cdot \vec{v}_1 + \\
 2 \hat{n} \cdot \vec{S}_1 \vec{S}_1 \cdot \vec{v}_1 \vec{v}_1 \cdot \vec{v}_1 - \frac{5}{2} \hat{n} \cdot \vec{S}_1 \vec{S}_1 \cdot \vec{a}_1 \vec{v}_1 \cdot \vec{v}_2 + \frac{5}{2} \hat{n} \cdot \vec{a}_1 \vec{S}_1 \cdot \vec{S}_1 \vec{v}_1 \cdot \vec{v}_2 - \frac{5}{2} \hat{n} \cdot \vec{S}_1 \vec{S}_1 \cdot \vec{v}_1 \vec{v}_1 \cdot \vec{v}_2 \Big) + \frac{1}{\rho^4} \\
 \left( -\frac{33}{4} \vec{S}_1 \cdot \vec{S}_1 \left( \hat{n} \cdot \vec{v}_1 \right)^4 + 18 \hat{n} \cdot \vec{v}_2 \vec{S}_1 \cdot \vec{S}_1 \left( \hat{n} \cdot \vec{v}_1 \right)^3 + \frac{33}{4} \hat{n} \cdot \vec{S}_1 \vec{S}_1 \cdot \vec{v}_1 \left( \hat{n} \cdot \vec{v}_1 \right)^3 + \frac{3}{4} \left( \hat{n} \times \vec{S}_1 \cdot \vec{v}_1 \right)^2 \left( \hat{n} \cdot \vec{v}_1 \right)^2 - \right. \\
 4 \left( \vec{S}_1 \cdot \vec{v}_1 \right)^2 \left( \hat{n} \cdot \vec{v}_1 \right)^2 - 18 \hat{n} \cdot \vec{S}_1 \hat{n} \cdot \vec{v}_2 \vec{S}_1 \cdot \vec{v}_1 \left( \hat{n} \cdot \vec{v}_1 \right)^2 + 3 \vec{S}_1 \cdot \vec{v}_1 \vec{S}_1 \cdot \vec{v}_2 \left( \hat{n} \cdot \vec{v}_1 \right)^2 + \frac{37}{4} \vec{S}_1 \cdot \vec{S}_1 \vec{v}_1 \cdot \vec{v}_1 \left( \hat{n} \cdot \vec{v}_1 \right)^2 - \\
 9 \vec{S}_1 \cdot \vec{S}_1 \vec{v}_1 \cdot \vec{v}_2 \left( \hat{n} \cdot \vec{v}_1 \right)^2 + 2 \hat{n} \cdot \vec{v}_2 \left( \vec{S}_1 \cdot \vec{v}_1 \right)^2 \hat{n} \cdot \vec{v}_1 + 8 \hat{n} \times \vec{S}_1 \cdot \vec{v}_1 \vec{S}_1 \times \vec{v}_1 \cdot \vec{v}_2 \hat{n} \cdot \vec{v}_1 - 24 \left( \hat{n} \times \vec{S}_1 \cdot \vec{v}_1 \right)^2 \hat{n} \cdot \vec{v}_2 \hat{n} \cdot \vec{v}_1 - \\
 4 \hat{n} \cdot \vec{v}_2 \vec{S}_1 \cdot \vec{S}_1 \vec{v}_1 \cdot \vec{v}_1 \hat{n} \cdot \vec{v}_1 - \frac{21}{4} \hat{n} \cdot \vec{S}_1 \vec{S}_1 \cdot \vec{v}_1 \vec{v}_1 \cdot \vec{v}_1 \hat{n} \cdot \vec{v}_1 + 6 \hat{n} \cdot \vec{S}_1 \vec{S}_1 \cdot \vec{v}_1 \vec{v}_1 \cdot \vec{v}_2 \hat{n} \cdot \vec{v}_1 - \\
 \vec{S}_1 \cdot \vec{S}_1 \left( \vec{v}_1 \cdot \vec{v}_1 \right)^2 - \frac{5}{4} \left( \hat{n} \times \vec{S}_1 \cdot \vec{v}_1 \right)^2 \vec{v}_1 \cdot \vec{v}_1 + \left( \vec{S}_1 \cdot \vec{v}_1 \right)^2 \vec{v}_1 \cdot \vec{v}_1 + 2 \hat{n} \cdot \vec{S}_1 \hat{n} \cdot \vec{v}_2 \vec{S}_1 \cdot \vec{v}_1 \vec{v}_1 \cdot \vec{v}_1 - \\
 \left. \frac{1}{2} \vec{S}_1 \cdot \vec{v}_1 \vec{S}_1 \cdot \vec{v}_2 \vec{v}_1 \cdot \vec{v}_1 + 4 \left( \hat{n} \times \vec{S}_1 \cdot \vec{v}_1 \right)^2 \vec{v}_1 \cdot \vec{v}_2 - \frac{1}{2} \left( \vec{S}_1 \cdot \vec{v}_1 \right)^2 \vec{v}_1 \cdot \vec{v}_2 + \vec{S}_1 \cdot \vec{S}_1 \vec{v}_1 \cdot \vec{v}_1 \vec{v}_1 \cdot \vec{v}_2 \right) \Big) m_2 \Big\}
 \end{aligned}$$

{DiagS1S1[2, 2, 23],

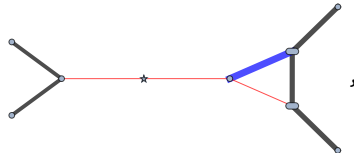

,

$$\begin{aligned}
 G^2 \left( \frac{1}{\rho^3} \left( 12 \hat{n} \cdot \vec{v}_2 \vec{S}_1 \cdot \vec{S}_1 \left( \hat{n} \cdot \vec{v}_1 \right)^2 - 6 \hat{n} \cdot \vec{S}_1 \hat{n} \cdot \vec{v}_2 \vec{S}_1 \cdot \vec{v}_1 \hat{n} \cdot \vec{v}_1 - 6 \hat{n} \cdot \vec{S}_1 \hat{n} \cdot \vec{v}_2 \vec{S}_1 \cdot \vec{a}_1 \hat{n} \cdot \vec{v}_1 + \right. \right. \\
 \left. 12 \hat{n} \cdot \vec{a}_1 \hat{n} \cdot \vec{v}_2 \vec{S}_1 \cdot \vec{S}_1 \hat{n} \cdot \vec{v}_1 - 3 \vec{a}_1 \cdot \vec{v}_2 \vec{S}_1 \cdot \vec{S}_1 \hat{n} \cdot \vec{v}_1 - 6 \hat{n} \cdot \vec{S}_1 \hat{n} \cdot \vec{v}_2 \vec{S}_1 \cdot \vec{v}_1 \hat{n} \cdot \vec{v}_1 + \frac{3}{2} \vec{S}_1 \cdot \vec{v}_2 \vec{S}_1 \cdot \vec{v}_1 \hat{n} \cdot \vec{v}_1 + \right.
 \end{aligned}$$

gS1S1[2, 2, 24],

$$G^2 \left( \frac{7}{r^2} \left( \frac{7}{2} \vec{v}_1 \cdot \vec{v}_2 \left( \hat{n} \cdot \vec{S}_1 \right)^2 - \frac{3}{2} \hat{n} \cdot \vec{v}_2 \vec{S}_1 \cdot \vec{v}_1 \hat{n} \cdot \vec{S}_1 - 3 \hat{n} \cdot \vec{v}_1 \vec{S}_1 \cdot \vec{v}_2 \hat{n} \cdot \vec{S}_1 + \frac{7}{2} \hat{n} \cdot \vec{S}_1 \vec{a}_1 \cdot \vec{v}_2 \hat{n} \cdot \vec{S}_1 - 4 \hat{n} \cdot \vec{v}_1 \vec{S}_1 \cdot \vec{a}_2 \hat{n} \cdot \vec{S}_1 - \right. \right.$$
$$\left. 4 \hat{n} \cdot \vec{a}_1 \vec{S}_1 \cdot \vec{v}_2 \hat{n} \cdot \vec{S}_1 + \frac{7}{2} \hat{n} \cdot \vec{S}_1 \vec{v}_1 \cdot \vec{a}_2 \hat{n} \cdot \vec{S}_1 + 3 \hat{n} \times \vec{S}_1 \cdot \vec{v}_1 \hat{n} \times \vec{S}_1 \cdot \vec{v}_2 + \frac{11}{2} \hat{n} \times \vec{S}_1 \cdot \vec{v}_2 \hat{n} \times \vec{S}_1 \cdot \vec{a}_1 - \right.$$
$$\left. \frac{5}{2} \hat{n} \times \vec{S}_1 \cdot \vec{v}_1 \hat{n} \times \vec{S}_1 \cdot \vec{a}_2 + \frac{11}{2} \hat{n} \times \vec{S}_1 \cdot \vec{a}_2 \hat{n} \times \vec{S}_1 \cdot \vec{v}_1 - \frac{5}{2} \hat{n} \times \vec{S}_1 \cdot \vec{a}_1 \hat{n} \times \vec{S}_1 \cdot \vec{v}_2 + \frac{9}{2} \hat{n} \cdot \vec{v}_1 \hat{n} \cdot \vec{v}_2 \vec{S}_1 \cdot \vec{S}_1 - \right.$$
$$\left. \frac{3}{2} \hat{n} \cdot \vec{S}_1 \hat{n} \cdot \vec{v}_2 \vec{S}_1 \cdot \vec{a}_1 + \hat{n} \cdot \vec{S}_1 \hat{n} \cdot \vec{v}_1 \vec{S}_1 \cdot \vec{a}_2 - \frac{3}{2} \hat{n} \cdot \vec{a}_2 \hat{n} \cdot \vec{S}_1 \vec{S}_1 \cdot \vec{v}_1 + \hat{n} \cdot \vec{a}_1 \hat{n} \cdot \vec{S}_1 \vec{S}_1 \cdot \vec{v}_2 + \right.$$
$$\left. \frac{7}{2} \vec{S}_1 \cdot \vec{v}_1 \vec{S}_1 \cdot \vec{v}_2 + \frac{9}{2} \hat{n} \cdot \vec{a}_2 \hat{n} \cdot \vec{v}_1 \vec{S}_1 \cdot \vec{S}_1 + \frac{9}{2} \hat{n} \cdot \vec{a}_1 \hat{n} \cdot \vec{v}_2 \vec{S}_1 \cdot \vec{S}_1 - 4 \vec{a}_1 \cdot \vec{v}_2 \vec{S}_1 \cdot \vec{S}_1 - \frac{3}{2} \vec{S}_1 \cdot \vec{v}_2 \vec{S}_1 \cdot \vec{a}_1 + \right.$$
$$\left. 5 \vec{S}_1 \cdot \vec{v}_1 \vec{S}_1 \cdot \vec{a}_2 - \frac{3}{2} \vec{S}_1 \cdot \vec{a}_2 \vec{S}_1 \cdot \vec{v}_1 + 5 \vec{S}_1 \cdot \vec{a}_1 \vec{S}_1 \cdot \vec{v}_2 - 4 \vec{S}_1 \cdot \vec{S}_1 \vec{v}_1 \cdot \vec{a}_2 - 4 \vec{S}_1 \cdot \vec{S}_1 \vec{v}_1 \cdot \vec{v}_2 \right) + \frac{1}{r^3}$$
$$\left( - (\hat{n} \cdot \vec{a}_2) \left( \hat{n} \times \vec{S}_1 \cdot \vec{v}_1 \right)^2 - \frac{3}{2} \vec{S}_1 \times \vec{v}_1 \cdot \vec{v}_2 \hat{n} \times \vec{S}_1 \cdot \vec{v}_1 + \frac{3}{2} \vec{S}_1 \times \vec{a}_1 \cdot \vec{v}_2 \hat{n} \times \vec{S}_1 \cdot \vec{v}_1 + 4 \hat{n} \times \vec{S}_1 \cdot \vec{v}_2 \hat{n} \cdot \vec{a}_1 \hat{n} \times \vec{S}_1 \cdot \vec{v}_1 - \right.$$
$$\left. 17 \hat{n} \times \vec{S}_1 \cdot \vec{v}_2 \hat{n} \cdot \vec{v}_1 \hat{n} \times \vec{S}_1 \cdot \vec{v}_1 + \hat{n} \times \vec{S}_1 \cdot \vec{a}_2 \hat{n} \cdot \vec{v}_1 \hat{n} \times \vec{S}_1 \cdot \vec{v}_1 + 22 \hat{n} \times \vec{S}_1 \cdot \vec{v}_2 \hat{n} \cdot \vec{v}_2 \hat{n} \times \vec{S}_1 \cdot \vec{v}_1 - \right.$$
$$\left. \hat{n} \times \vec{S}_1 \cdot \vec{a}_1 \hat{n} \cdot \vec{v}_2 \hat{n} \times \vec{S}_1 \cdot \vec{v}_1 - \frac{1}{2} \hat{n} \cdot \vec{a}_2 \left( \vec{S}_1 \cdot \vec{v}_1 \right)^2 + \frac{5}{2} \hat{n} \times \vec{S}_1 \cdot \vec{v}_2 \vec{S}_1 \times \vec{v}_1 \cdot \vec{v}_2 - \frac{3}{2} \hat{n} \times \vec{S}_1 \cdot \vec{v}_2 \vec{S}_1 \times \vec{v}_1 \cdot \vec{a}_1 - \right.$$
$$\left. \frac{3}{2} \hat{n} \times \vec{S}_1 \cdot \vec{v}_1 \vec{S}_1 \times \vec{v}_1 \cdot \vec{v}_2 - \frac{11}{2} \hat{n} \times \vec{S}_1 \cdot \vec{v}_2 \vec{S}_1 \times \vec{v}_1 \cdot \vec{v}_2 - \frac{3}{2} \hat{n} \times \vec{S}_1 \cdot \vec{a}_1 \vec{S}_1 \times \vec{v}_1 \cdot \vec{v}_2 + 5 \hat{n} \times \vec{S}_1 \cdot \vec{v}_1 \hat{n} \times \vec{S}_1 \cdot \vec{v}_2 \hat{n} \cdot \vec{v}_1 - \right.$$
$$\left. 3 \hat{n} \times \vec{S}_1 \cdot \vec{a}_1 \hat{n} \times \vec{S}_1 \cdot \vec{v}_2 \hat{n} \cdot \vec{v}_1 - 10 \hat{n} \times \vec{S}_1 \cdot \vec{v}_1 \hat{n} \times \vec{S}_1 \cdot \vec{v}_2 \hat{n} \cdot \vec{v}_2 - 6 \hat{n} \cdot \vec{S}_1 \left( \hat{n} \cdot \vec{v}_2 \right)^2 \vec{S}_1 \cdot \vec{v}_1 + \right.$$
$$\left. 3 \hat{n} \cdot \vec{S}_1 \hat{n} \cdot \vec{v}_1 \hat{n} \cdot \vec{v}_2 \vec{S}_1 \cdot \vec{v}_1 + 2 \hat{n} \cdot \vec{S}_1 \left( \hat{n} \cdot \vec{v}_1 \right)^2 \vec{S}_1 \cdot \vec{v}_2 + 4 \hat{n} \cdot \vec{S}_1 \hat{n} \cdot \vec{v}_1 \hat{n} \cdot \vec{v}_2 \vec{S}_1 \cdot \vec{v}_2 - 4 \left( \hat{n} \cdot \vec{S}_1 \right)^2 \hat{n} \cdot \vec{v}_1 \vec{a}_1 \cdot \vec{v}_2 + \right.$$
$$\left. 18 \hat{n} \cdot \vec{v}_1 \left( \hat{n} \cdot \vec{v}_2 \right)^2 \vec{S}_1 \cdot \vec{S}_1 - 18 \left( \hat{n} \cdot \vec{v}_1 \right)^2 \hat{n} \cdot \vec{v}_2 \vec{S}_1 \cdot \vec{S}_1 + 3 \hat{n} \cdot \vec{S}_1 \hat{n} \cdot \vec{v}_1 \hat{n} \cdot \vec{v}_2 \vec{S}_1 \cdot \vec{a}_1 + 2 \hat{n} \cdot \vec{S}_1 \left( \hat{n} \cdot \vec{v}_1 \right)^2 \vec{S}_1 \cdot \vec{a}_2 - \right.$$
$$\left. 5 \hat{n} \cdot \vec{a}_2 \left( \hat{n} \cdot \vec{v}_1 \right)^2 \vec{S}_1 \cdot \vec{S}_1 - 5 \hat{n} \cdot \vec{a}_1 \hat{n} \cdot \vec{v}_1 \hat{n} \cdot \vec{v}_2 \vec{S}_1 \cdot \vec{S}_1 + \frac{3}{2} \hat{n} \cdot \vec{v}_1 \vec{a}_1 \cdot \vec{v}_2 \vec{S}_1 \cdot \vec{S}_1 + 3 \hat{n} \cdot \vec{a}_2 \hat{n} \cdot \vec{S}_1 \hat{n} \cdot \vec{v}_1 \vec{S}_1 \cdot \vec{v}_1 + \right.$$
$$\left. 3 \hat{n} \cdot \vec{S}_1 \hat{n} \cdot \vec{v}_1 \hat{n} \cdot \vec{v}_2 \vec{S}_1 \cdot \vec{v}_1 - \frac{3}{2} \hat{n} \cdot \vec{v}_2 \vec{S}_1 \cdot \vec{v}_1 \vec{S}_1 \cdot \vec{v}_1 - \hat{n} \cdot \vec{v}_1 \vec{S}_1 \cdot \vec{v}_2 \vec{S}_1 \cdot \vec{v}_1 - 3 \hat{n} \cdot \vec{v}_2 \vec{S}_1 \cdot \vec{v}_2 \vec{S}_1 \cdot \vec{v}_1 + \right.$$
$$\left. \frac{5}{2} \hat{n} \cdot \vec{S}_1 \vec{a}_1 \cdot \vec{v}_2 \vec{S}_1 \cdot \vec{v}_1 - \frac{1}{2} \hat{n} \cdot \vec{v}_2 \vec{S}_1 \cdot \vec{a}_1 \vec{S}_1 \cdot \vec{v}_1 - 2 \hat{n} \cdot \vec{v}_1 \vec{S}_1 \cdot \vec{a}_2 \vec{S}_1 \cdot \vec{v}_1 + 10 \hat{n} \cdot \vec{S}_1 \left( \hat{n} \cdot \vec{v}_1 \right)^2 \vec{S}_1 \cdot \vec{v}_2 + \right.$$

[illegible]

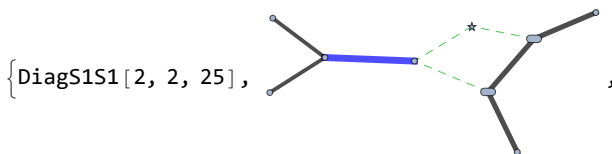

$$G^2 \left( \frac{1}{r^2} \left( \frac{5}{2} \left( \hat{n} \times \vec{S}_1 \cdot \vec{v}_2 \right)^2 + \frac{5}{2} \hat{n} \times \vec{S}_1 \cdot \vec{a}_2 \hat{n} \times \vec{S}_1 \cdot \vec{v}_2 + \frac{1}{3} \left( \hat{n} \cdot \vec{S}_1 \right)^2 \left( \hat{n} \cdot \vec{v}_2 \right)^2 + \frac{11}{6} \left( \vec{S}_1 \cdot \vec{v}_2 \right)^2 + \frac{5}{2} \hat{n} \times \vec{S}_1 \cdot \vec{a}_2 \hat{n} \times \vec{S}_1 \cdot \vec{v}_2 + \right. \right. \\ \left. \frac{2}{3} \hat{n} \cdot \vec{S}_1 \hat{n} \cdot \vec{a}_2 \hat{n} \cdot \vec{S}_1 \hat{n} \cdot \vec{v}_2 + \frac{8}{3} \left( \hat{n} \cdot \vec{v}_2 \right)^2 \vec{S}_1 \cdot \vec{S}_1 - \frac{2}{3} \hat{n} \cdot \vec{S}_1 \hat{n} \cdot \vec{v}_2 \vec{S}_1 \cdot \vec{a}_2 - \frac{2}{3} \hat{n} \cdot \vec{a}_2 \hat{n} \cdot \vec{S}_1 \vec{S}_1 \cdot \vec{v}_2 - \right. \\ \left. \frac{10}{3} \hat{n} \cdot \vec{S}_1 \hat{n} \cdot \vec{v}_2 \vec{S}_1 \cdot \vec{v}_2 + \frac{16}{3} \hat{n} \cdot \vec{a}_2 \hat{n} \cdot \vec{v}_2 \vec{S}_1 \cdot \vec{S}_1 - \frac{8}{3} \hat{n} \cdot \vec{S}_1 \hat{n} \cdot \vec{v}_2 \vec{S}_1 \cdot \vec{a}_2 + \frac{11}{6} \vec{S}_1 \cdot \vec{v}_2 \vec{S}_1 \cdot \vec{a}_2 - \frac{8}{3} \hat{n} \cdot \vec{S}_1 \hat{n} \cdot \vec{a}_2 \vec{S}_1 \cdot \vec{v}_2 + \right.$$



$$\frac{7}{4} \left( \hat{n} \cdot \vec{S}_1 \right)^2 \vec{v}_1 \cdot \vec{v}_1 \vec{v}_2 \cdot \vec{v}_2 - \frac{1}{2} \vec{S}_1 \cdot \vec{S}_1 \vec{v}_1 \cdot \vec{v}_1 \vec{v}_2 \cdot \vec{v}_2 + \frac{7}{4} \left( \hat{n} \cdot \vec{S}_1 \right)^2 \vec{v}_1 \cdot \vec{v}_2 \vec{v}_2 \cdot \vec{v}_2 - \frac{9}{4} \vec{S}_1 \cdot \vec{S}_1 \vec{v}_1 \cdot \vec{v}_2 \vec{v}_2 \cdot \vec{v}_2 \right) m_2 \}$$

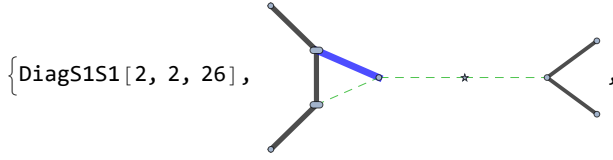

$$\begin{aligned} G^2 \left( \frac{1}{r^2} \left( -\frac{1}{2} \vec{a}_1 \cdot \vec{a}_2 \left( \hat{n} \cdot \vec{S}_1 \right)^2 + \hat{n} \cdot \vec{v}_1 \vec{S}_1 \cdot \vec{a}_2 \hat{n} \cdot \vec{S}_1 + \frac{3}{2} \hat{n} \cdot \vec{a}_2 \vec{S}_1 \cdot \vec{v}_1 \hat{n} \cdot \vec{S}_1 + \frac{3}{2} \hat{n} \cdot \vec{a}_2 \vec{S}_1 \cdot \vec{a}_1 \hat{n} \cdot \vec{S}_1 + \hat{n} \cdot \vec{a}_1 \vec{S}_1 \cdot \vec{a}_2 \hat{n} \cdot \vec{S}_1 - \right. \right. \\ \left. \hat{n} \cdot \vec{S}_1 \vec{v}_1 \cdot \vec{a}_2 \hat{n} \cdot \vec{S}_1 - 5 \hat{n} \cdot \vec{a}_2 \hat{n} \cdot \vec{v}_1 \vec{S}_1 \cdot \vec{S}_1 + \hat{n} \cdot \vec{S}_1 \hat{n} \cdot \vec{v}_1 \vec{S}_1 \cdot \vec{a}_2 - \vec{S}_1 \cdot \vec{v}_1 \vec{S}_1 \cdot \vec{a}_2 - \vec{S}_1 \cdot \vec{a}_1 \vec{S}_1 \cdot \vec{a}_2 - \right. \\ \left. \frac{5}{2} \hat{n} \cdot \vec{a}_1 \hat{n} \cdot \vec{a}_2 \vec{S}_1 \cdot \vec{S}_1 + \frac{3}{2} \vec{a}_1 \cdot \vec{a}_2 \vec{S}_1 \cdot \vec{S}_1 + \frac{3}{2} \hat{n} \cdot \vec{S}_1 \hat{n} \cdot \vec{a}_2 \vec{S}_1 \cdot \vec{v}_1 - \vec{S}_1 \cdot \vec{a}_2 \vec{S}_1 \cdot \vec{v}_1 + 3 \vec{S}_1 \cdot \vec{S}_1 \vec{v}_1 \cdot \vec{a}_2 \right) + \frac{1}{r^3} \\ \left( -2 \hat{n} \cdot \vec{v}_2 \vec{a}_1 \cdot \vec{v}_2 \left( \hat{n} \cdot \vec{S}_1 \right)^2 + 2 \hat{n} \cdot \vec{v}_1 \vec{v}_1 \cdot \vec{a}_2 \left( \hat{n} \cdot \vec{S}_1 \right)^2 + 6 \left( \hat{n} \cdot \vec{v}_2 \right)^2 \vec{S}_1 \cdot \vec{v}_1 \hat{n} \cdot \vec{S}_1 + 4 \hat{n} \cdot \vec{v}_1 \hat{n} \cdot \vec{v}_2 \vec{S}_1 \cdot \vec{v}_2 \hat{n} \cdot \vec{S}_1 + \right. \\ \left. 6 \left( \hat{n} \cdot \vec{v}_2 \right)^2 \vec{S}_1 \cdot \vec{a}_1 \hat{n} \cdot \vec{S}_1 - 4 \left( \hat{n} \cdot \vec{v}_1 \right)^2 \vec{S}_1 \cdot \vec{a}_2 \hat{n} \cdot \vec{S}_1 - 6 \hat{n} \cdot \vec{a}_2 \hat{n} \cdot \vec{v}_1 \vec{S}_1 \cdot \vec{v}_1 \hat{n} \cdot \vec{S}_1 + 4 \hat{n} \cdot \vec{a}_1 \hat{n} \cdot \vec{v}_2 \vec{S}_1 \cdot \vec{v}_2 \hat{n} \cdot \vec{S}_1 + \right. \\ \left. \frac{1}{2} \vec{S}_1 \cdot \vec{v}_1 \vec{v}_1 \cdot \vec{a}_2 \hat{n} \cdot \vec{S}_1 + \vec{S}_1 \cdot \vec{a}_2 \vec{v}_1 \cdot \vec{v}_1 \hat{n} \cdot \vec{S}_1 - 4 \hat{n} \cdot \vec{S}_1 \hat{n} \cdot \vec{v}_2 \vec{v}_1 \cdot \vec{v}_2 \hat{n} \cdot \vec{S}_1 - \frac{3}{2} \vec{S}_1 \cdot \vec{v}_1 \vec{v}_2 \cdot \vec{v}_2 \hat{n} \cdot \vec{S}_1 - \right. \\ \left. \frac{3}{2} \vec{S}_1 \cdot \vec{a}_1 \vec{v}_2 \cdot \vec{v}_2 \hat{n} \cdot \vec{S}_1 + \frac{3}{2} \hat{n} \cdot \vec{a}_2 \left( \vec{S}_1 \cdot \vec{v}_1 \right)^2 - \hat{n} \cdot \vec{a}_1 \left( \vec{S}_1 \cdot \vec{v}_2 \right)^2 - 20 \hat{n} \cdot \vec{v}_1 \left( \hat{n} \cdot \vec{v}_2 \right)^2 \vec{S}_1 \cdot \vec{S}_1 + \right. \\ \left. 10 \hat{n} \cdot \vec{a}_2 \left( \hat{n} \cdot \vec{v}_1 \right)^2 \vec{S}_1 \cdot \vec{S}_1 - 10 \hat{n} \cdot \vec{a}_1 \left( \hat{n} \cdot \vec{v}_2 \right)^2 \vec{S}_1 \cdot \vec{S}_1 + \frac{11}{2} \hat{n} \cdot \vec{v}_2 \vec{a}_1 \cdot \vec{v}_2 \vec{S}_1 \cdot \vec{S}_1 + 6 \hat{n} \cdot \vec{S}_1 \left( \hat{n} \cdot \vec{v}_2 \right)^2 \vec{S}_1 \cdot \vec{v}_1 - \right. \\ \left. \frac{7}{2} \hat{n} \cdot \vec{v}_2 \vec{S}_1 \cdot \vec{v}_2 \vec{S}_1 \cdot \vec{v}_1 + 3 \hat{n} \cdot \vec{v}_1 \vec{S}_1 \cdot \vec{a}_2 \vec{S}_1 \cdot \vec{v}_1 + 4 \hat{n} \cdot \vec{S}_1 \hat{n} \cdot \vec{v}_1 \hat{n} \cdot \vec{v}_2 \vec{S}_1 \cdot \vec{v}_2 - \frac{7}{2} \hat{n} \cdot \vec{v}_2 \vec{S}_1 \cdot \vec{v}_1 \vec{S}_1 \cdot \vec{v}_2 - \right. \\ \left. 2 \hat{n} \cdot \vec{v}_1 \vec{S}_1 \cdot \vec{v}_2 \vec{S}_1 \cdot \vec{v}_2 - \frac{7}{2} \hat{n} \cdot \vec{v}_2 \vec{S}_1 \cdot \vec{a}_1 \vec{S}_1 \cdot \vec{v}_2 - \frac{11}{2} \hat{n} \cdot \vec{v}_1 \vec{S}_1 \cdot \vec{S}_1 \vec{v}_1 \cdot \vec{a}_2 - \frac{5}{2} \hat{n} \cdot \vec{a}_2 \vec{S}_1 \cdot \vec{S}_1 \vec{v}_1 \cdot \vec{v}_1 + \right. \\ \left. 11 \hat{n} \cdot \vec{v}_2 \vec{S}_1 \cdot \vec{S}_1 \vec{v}_1 \cdot \vec{v}_2 + 5 \hat{n} \cdot \vec{v}_1 \vec{S}_1 \cdot \vec{S}_1 \vec{v}_2 \cdot \vec{v}_2 + \frac{5}{2} \hat{n} \cdot \vec{a}_1 \vec{S}_1 \cdot \vec{S}_1 \vec{v}_2 \cdot \vec{v}_2 - \frac{3}{2} \hat{n} \cdot \vec{S}_1 \vec{S}_1 \cdot \vec{v}_1 \vec{v}_2 \cdot \vec{v}_2 \right) + \\ \frac{1}{r^4} \left( -2 \left( \vec{v}_1 \cdot \vec{v}_2 \right)^2 \left( \hat{n} \cdot \vec{S}_1 \right)^2 + 12 \hat{n} \cdot \vec{v}_1 \hat{n} \cdot \vec{v}_2 \vec{v}_1 \cdot \vec{v}_2 \left( \hat{n} \cdot \vec{S}_1 \right)^2 - 36 \hat{n} \cdot \vec{v}_1 \left( \hat{n} \cdot \vec{v}_2 \right)^2 \vec{S}_1 \cdot \vec{v}_1 \hat{n} \cdot \vec{S}_1 - \right. \\ \left. 24 \left( \hat{n} \cdot \vec{v}_1 \right)^2 \hat{n} \cdot \vec{v}_2 \vec{S}_1 \cdot \vec{v}_2 \hat{n} \cdot \vec{S}_1 + 4 \hat{n} \cdot \vec{v}_2 \vec{S}_1 \cdot \vec{v}_2 \vec{v}_1 \cdot \vec{v}_1 \hat{n} \cdot \vec{S}_1 + 8 \hat{n} \cdot \vec{v}_2 \vec{S}_1 \cdot \vec{v}_1 \vec{v}_1 \cdot \vec{v}_2 \hat{n} \cdot \vec{S}_1 + \right. \\ \left. 4 \hat{n} \cdot \vec{v}_1 \vec{S}_1 \cdot \vec{v}_2 \vec{v}_1 \cdot \vec{v}_2 \hat{n} \cdot \vec{S}_1 + 6 \hat{n} \cdot \vec{v}_1 \vec{S}_1 \cdot \vec{v}_1 \vec{v}_2 \cdot \vec{v}_2 \hat{n} \cdot \vec{S}_1 + 6 \left( \hat{n} \cdot \vec{v}_2 \right)^2 \left( \vec{S}_1 \cdot \vec{v}_1 \right)^2 + 4 \left( \hat{n} \cdot \vec{v}_1 \right)^2 \left( \vec{S}_1 \cdot \vec{v}_2 \right)^2 + \right. \\ \left. \frac{11}{2} \vec{S}_1 \cdot \vec{S}_1 \left( \vec{v}_1 \cdot \vec{v}_2 \right)^2 + 60 \left( \hat{n} \cdot \vec{v}_1 \right)^2 \left( \hat{n} \cdot \vec{v}_2 \right)^2 \vec{S}_1 \cdot \vec{S}_1 + 18 \hat{n} \cdot \vec{v}_1 \hat{n} \cdot \vec{v}_2 \vec{S}_1 \cdot \vec{v}_1 \vec{S}_1 \cdot \vec{v}_2 - \right. \\ \left. \left( \vec{S}_1 \cdot \vec{v}_2 \right)^2 \vec{v}_1 \cdot \vec{v}_1 - 10 \left( \hat{n} \cdot \vec{v}_2 \right)^2 \vec{S}_1 \cdot \vec{S}_1 \vec{v}_1 \cdot \vec{v}_1 - 42 \hat{n} \cdot \vec{v}_1 \hat{n} \cdot \vec{v}_2 \vec{S}_1 \cdot \vec{S}_1 \vec{v}_1 \cdot \vec{v}_2 - \frac{7}{2} \vec{S}_1 \cdot \vec{v}_1 \vec{S}_1 \cdot \vec{v}_2 \vec{v}_1 \cdot \vec{v}_2 - \right. \\ \left. \frac{3}{2} \left( \vec{S}_1 \cdot \vec{v}_1 \right)^2 \vec{v}_2 \cdot \vec{v}_2 - 10 \left( \hat{n} \cdot \vec{v}_1 \right)^2 \vec{S}_1 \cdot \vec{S}_1 \vec{v}_2 \cdot \vec{v}_2 + \frac{5}{2} \vec{S}_1 \cdot \vec{S}_1 \vec{v}_1 \cdot \vec{v}_1 \vec{v}_2 \cdot \vec{v}_2 \right) \Big) m_2 \} \end{aligned}$$

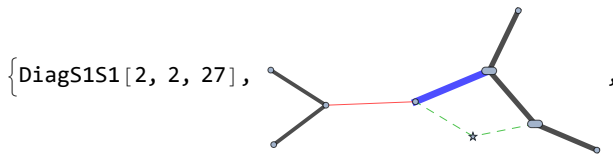

$$\begin{aligned} G^2 \left( \frac{1}{r} \left( \frac{2}{3} \hat{n} \cdot \vec{S}_1 \hat{n} \cdot \vec{a}_1 \hat{n} \cdot \vec{S}_1 - \frac{1}{3} \vec{S}_1 \cdot \vec{a}_1 \hat{n} \cdot \vec{S}_1 + \frac{2}{3} \hat{n} \cdot \vec{S}_1 \hat{n} \cdot \vec{S}_1 \hat{n} \cdot \vec{v}_1 - \right. \right. \\ \left. \frac{7}{3} \hat{n} \cdot \vec{v}_1 \vec{S}_1 \cdot \vec{S}_1 + \frac{2}{3} \hat{n} \cdot \vec{S}_1 \vec{S}_1 \cdot \vec{v}_1 - \frac{1}{3} \hat{n} \cdot \vec{S}_1 \vec{S}_1 \cdot \vec{v}_1 - \frac{7}{3} \hat{n} \cdot \vec{a}_1 \vec{S}_1 \cdot \vec{S}_1 + \frac{2}{3} \hat{n} \cdot \vec{S}_1 \vec{S}_1 \cdot \vec{a}_1 \right) + \frac{1}{r^2} \\ \left( - \left( \hat{n} \times \vec{S}_1 \cdot \vec{v}_1 \right)^2 - \frac{1}{2} \left( \hat{n} \times \vec{S}_1 \cdot \vec{a}_1 \right)^2 - \frac{2}{3} \left( \hat{n} \cdot \vec{a}_1 \right)^2 \left( \hat{n} \cdot \vec{S}_1 \right)^2 - \frac{4}{3} \left( \hat{n} \cdot \vec{S}_1 \right)^2 \left( \hat{n} \cdot \vec{v}_1 \right)^2 - 2 \hat{n} \cdot \vec{S}_1 \hat{n} \cdot \vec{S}_1 \left( \hat{n} \cdot \vec{v}_1 \right)^2 - \right. \end{aligned}$$





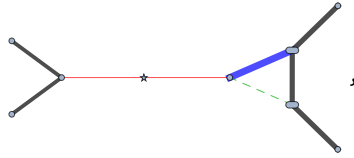

[illegible]

$$\begin{aligned}
& \frac{28}{3} \hat{n} \cdot \vec{a}_1 (\hat{n} \cdot \vec{v}_2)^2 \vec{S}_1 \cdot \vec{S}_1 - \frac{44}{3} \hat{n} \cdot \vec{a}_1 \hat{n} \cdot \vec{v}_1 \hat{n} \cdot \vec{v}_2 \vec{S}_1 \cdot \vec{S}_1 + \frac{11}{3} \hat{n} \cdot \vec{v}_1 \vec{a}_1 \cdot \vec{v}_2 \vec{S}_1 \cdot \vec{S}_1 - \frac{14}{3} \hat{n} \cdot \vec{v}_2 \vec{a}_1 \cdot \vec{v}_2 \vec{S}_1 \cdot \vec{S}_1 - \\
& \frac{16}{3} \hat{n} \cdot \vec{S}_1 (\hat{n} \cdot \vec{v}_2)^2 \vec{S}_1 \cdot \vec{v}_1 + \frac{34}{3} \hat{n} \cdot \vec{S}_1 \hat{n} \cdot \vec{v}_1 \hat{n} \cdot \vec{v}_2 \vec{S}_1 \cdot \vec{v}_1 - \frac{7}{3} \hat{n} \cdot \vec{v}_2 \vec{S}_1 \cdot \vec{v}_1 \vec{S}_1 \cdot \vec{v}_1 - \frac{17}{6} \hat{n} \cdot \vec{v}_1 \vec{S}_1 \cdot \vec{v}_2 \vec{S}_1 \cdot \vec{v}_1 + \\
& \frac{8}{3} \hat{n} \cdot \vec{v}_2 \vec{S}_1 \cdot \vec{v}_2 \vec{S}_1 \cdot \vec{v}_1 - \frac{2}{3} \hat{n} \cdot \vec{v}_2 \vec{S}_1 \cdot \vec{a}_1 \vec{S}_1 \cdot \vec{v}_1 - \frac{5}{3} \hat{n} \cdot \vec{v}_1 \vec{S}_1 \cdot \vec{a}_2 \vec{S}_1 \cdot \vec{v}_1 + \frac{8}{3} \hat{n} \cdot \vec{S}_1 (\hat{n} \cdot \vec{v}_1)^2 \vec{S}_1 \cdot \vec{v}_2 - \\
& \frac{8}{3} \hat{n} \cdot \vec{S}_1 \hat{n} \cdot \vec{v}_1 \hat{n} \cdot \vec{v}_2 \vec{S}_1 \cdot \vec{v}_2 - \frac{11}{6} \hat{n} \cdot \vec{v}_1 \vec{S}_1 \cdot \vec{v}_1 \vec{S}_1 \cdot \vec{v}_2 + \frac{8}{3} \hat{n} \cdot \vec{v}_2 \vec{S}_1 \cdot \vec{v}_1 \vec{S}_1 \cdot \vec{v}_2 + \frac{2}{3} \hat{n} \cdot \vec{v}_1 \vec{S}_1 \cdot \vec{v}_2 \vec{S}_1 \cdot \vec{v}_2 - \\
& \frac{7}{6} \hat{n} \cdot \vec{v}_1 \vec{S}_1 \cdot \vec{a}_1 \vec{S}_1 \cdot \vec{v}_2 + \frac{8}{3} \hat{n} \cdot \vec{v}_2 \vec{S}_1 \cdot \vec{a}_1 \vec{S}_1 \cdot \vec{v}_2 - \frac{7}{6} \hat{n} \cdot \vec{a}_1 \vec{S}_1 \cdot \vec{v}_1 \vec{S}_1 \cdot \vec{v}_2 + \frac{8}{3} \hat{n} \cdot \vec{v}_2 \vec{S}_1 \cdot \vec{S}_1 \vec{v}_1 \cdot \vec{a}_1 + \\
& \frac{14}{3} \hat{n} \cdot \vec{v}_1 \vec{S}_1 \cdot \vec{S}_1 \vec{v}_1 \cdot \vec{a}_2 + \frac{19}{3} \hat{n} \cdot \vec{v}_2 \vec{S}_1 \cdot \vec{S}_1 \vec{v}_1 \cdot \vec{v}_1 + \frac{7}{3} \hat{n} \cdot \vec{a}_2 \vec{S}_1 \cdot \vec{S}_1 \vec{v}_1 \cdot \vec{v}_1 - \frac{2}{3} \hat{n} \cdot \vec{S}_1 \vec{S}_1 \cdot \vec{v}_2 \vec{v}_1 \cdot \vec{v}_1 + \\
& \frac{44}{3} \hat{n} \cdot \vec{v}_1 \vec{S}_1 \cdot \vec{S}_1 \vec{v}_1 \cdot \vec{v}_2 - \frac{28}{3} \hat{n} \cdot \vec{v}_2 \vec{S}_1 \cdot \vec{S}_1 \vec{v}_1 \cdot \vec{v}_2 + \frac{11}{3} \hat{n} \cdot \vec{a}_1 \vec{S}_1 \cdot \vec{S}_1 \vec{v}_1 \cdot \vec{v}_2 - \frac{17}{6} \hat{n} \cdot \vec{S}_1 \vec{S}_1 \cdot \vec{v}_1 \vec{v}_1 \cdot \vec{v}_2 + \\
& \frac{2}{3} \hat{n} \cdot \vec{S}_1 \vec{S}_1 \cdot \vec{v}_2 \vec{v}_1 \cdot \vec{v}_2 - \frac{14}{3} \hat{n} \cdot \vec{v}_1 \vec{S}_1 \cdot \vec{S}_1 \vec{v}_2 \cdot \vec{v}_2 - \frac{7}{3} \hat{n} \cdot \vec{a}_1 \vec{S}_1 \cdot \vec{S}_1 \vec{v}_2 \cdot \vec{v}_2 + \frac{4}{3} \hat{n} \cdot \vec{S}_1 \vec{S}_1 \cdot \vec{v}_1 \vec{v}_2 \cdot \vec{v}_2 \Big) + \\
& \frac{1}{r^4} \Big( 32 (\hat{n} \cdot \vec{S}_1)^2 \hat{n} \cdot \vec{v}_2 (\hat{n} \cdot \vec{v}_1)^3 + 44 \hat{n} \cdot \vec{v}_2 \vec{S}_1 \cdot \vec{S}_1 (\hat{n} \cdot \vec{v}_1)^3 - 8 \hat{n} \cdot \vec{S}_1 \vec{S}_1 \cdot \vec{v}_2 (\hat{n} \cdot \vec{v}_1)^3 - \\
& 32 (\hat{n} \cdot \vec{S}_1)^2 (\hat{n} \cdot \vec{v}_2)^2 (\hat{n} \cdot \vec{v}_1)^2 - \frac{4}{3} (\vec{S}_1 \cdot \vec{v}_2)^2 (\hat{n} \cdot \vec{v}_1)^2 - 56 (\hat{n} \cdot \vec{v}_2)^2 \vec{S}_1 \cdot \vec{S}_1 (\hat{n} \cdot \vec{v}_1)^2 - \\
& 36 \hat{n} \cdot \vec{S}_1 \hat{n} \cdot \vec{v}_2 \vec{S}_1 \cdot \vec{v}_1 (\hat{n} \cdot \vec{v}_1)^2 + 16 \hat{n} \cdot \vec{S}_1 \hat{n} \cdot \vec{v}_2 \vec{S}_1 \cdot \vec{v}_2 (\hat{n} \cdot \vec{v}_1)^2 + 6 \vec{S}_1 \cdot \vec{v}_1 \vec{S}_1 \cdot \vec{v}_2 (\hat{n} \cdot \vec{v}_1)^2 - \\
& 12 (\hat{n} \cdot \vec{S}_1)^2 \vec{v}_1 \cdot \vec{v}_2 (\hat{n} \cdot \vec{v}_1)^2 - 22 \vec{S}_1 \cdot \vec{S}_1 \vec{v}_1 \cdot \vec{v}_2 (\hat{n} \cdot \vec{v}_1)^2 + 4 (\hat{n} \cdot \vec{S}_1)^2 \vec{v}_2 \cdot \vec{v}_2 (\hat{n} \cdot \vec{v}_1)^2 + \\
& \frac{28}{3} \vec{S}_1 \cdot \vec{S}_1 \vec{v}_2 \cdot \vec{v}_2 (\hat{n} \cdot \vec{v}_1)^2 + 6 \hat{n} \cdot \vec{v}_2 (\vec{S}_1 \cdot \vec{v}_1)^2 \hat{n} \cdot \vec{v}_1 + 4 \hat{n} \times \vec{S}_1 \cdot \vec{v}_1 \vec{S}_1 \times \vec{v}_1 \cdot \vec{v}_2 \hat{n} \cdot \vec{v}_1 - \\
& 12 (\hat{n} \times \vec{S}_1 \cdot \vec{v}_1)^2 \hat{n} \cdot \vec{v}_2 \hat{n} \cdot \vec{v}_1 + 40 \hat{n} \cdot \vec{S}_1 (\hat{n} \cdot \vec{v}_2)^2 \vec{S}_1 \cdot \vec{v}_1 \hat{n} \cdot \vec{v}_1 - \frac{40}{3} \hat{n} \cdot \vec{v}_2 \vec{S}_1 \cdot \vec{v}_1 \vec{S}_1 \cdot \vec{v}_2 \hat{n} \cdot \vec{v}_1 - \\
& 12 (\hat{n} \cdot \vec{S}_1)^2 \hat{n} \cdot \vec{v}_2 \vec{v}_1 \cdot \vec{v}_1 \hat{n} \cdot \vec{v}_1 - 20 \hat{n} \cdot \vec{v}_2 \vec{S}_1 \cdot \vec{S}_1 \vec{v}_1 \cdot \vec{v}_1 \hat{n} \cdot \vec{v}_1 + 4 \hat{n} \cdot \vec{S}_1 \vec{S}_1 \cdot \vec{v}_2 \vec{v}_1 \cdot \vec{v}_1 \hat{n} \cdot \vec{v}_1 + \\
& 16 (\hat{n} \cdot \vec{S}_1)^2 \hat{n} \cdot \vec{v}_2 \vec{v}_1 \cdot \vec{v}_2 \hat{n} \cdot \vec{v}_1 + \frac{112}{3} \hat{n} \cdot \vec{v}_2 \vec{S}_1 \cdot \vec{S}_1 \vec{v}_1 \cdot \vec{v}_2 \hat{n} \cdot \vec{v}_1 + 12 \hat{n} \cdot \vec{S}_1 \vec{S}_1 \cdot \vec{v}_1 \vec{v}_1 \cdot \vec{v}_2 \hat{n} \cdot \vec{v}_1 - \\
& \frac{16}{3} \hat{n} \cdot \vec{S}_1 \vec{S}_1 \cdot \vec{v}_2 \vec{v}_1 \cdot \vec{v}_2 \hat{n} \cdot \vec{v}_1 - \frac{20}{3} \hat{n} \cdot \vec{S}_1 \vec{S}_1 \cdot \vec{v}_1 \vec{v}_2 \cdot \vec{v}_2 \hat{n} \cdot \vec{v}_1 - \frac{16}{3} (\hat{n} \cdot \vec{v}_2)^2 (\vec{S}_1 \cdot \vec{v}_1)^2 - \frac{4}{3} (\hat{n} \cdot \vec{S}_1)^2 (\vec{v}_1 \cdot \vec{v}_2)^2 - \\
& \frac{14}{3} \vec{S}_1 \cdot \vec{S}_1 (\vec{v}_1 \cdot \vec{v}_2)^2 + 4 (\hat{n} \cdot \vec{S}_1)^2 (\hat{n} \cdot \vec{v}_2)^2 \vec{v}_1 \cdot \vec{v}_1 + \frac{1}{3} (\vec{S}_1 \cdot \vec{v}_2)^2 \vec{v}_1 \cdot \vec{v}_1 + \frac{28}{3} (\hat{n} \cdot \vec{v}_2)^2 \vec{S}_1 \cdot \vec{S}_1 \vec{v}_1 \cdot \vec{v}_1 + \\
& 6 \hat{n} \cdot \vec{S}_1 \hat{n} \cdot \vec{v}_2 \vec{S}_1 \cdot \vec{v}_1 \vec{v}_1 \cdot \vec{v}_1 - \frac{8}{3} \hat{n} \cdot \vec{S}_1 \hat{n} \cdot \vec{v}_2 \vec{S}_1 \cdot \vec{v}_2 \vec{v}_1 \cdot \vec{v}_1 - \frac{3}{2} \vec{S}_1 \cdot \vec{v}_1 \vec{S}_1 \cdot \vec{v}_2 \vec{v}_1 \cdot \vec{v}_1 + 2 (\hat{n} \times \vec{S}_1 \cdot \vec{v}_1)^2 \vec{v}_1 \cdot \vec{v}_2 - \\
& \frac{3}{2} (\vec{S}_1 \cdot \vec{v}_1)^2 \vec{v}_1 \cdot \vec{v}_2 - \frac{40}{3} \hat{n} \cdot \vec{S}_1 \hat{n} \cdot \vec{v}_2 \vec{S}_1 \cdot \vec{v}_1 \vec{v}_1 \cdot \vec{v}_2 + \frac{10}{3} \vec{S}_1 \cdot \vec{v}_1 \vec{S}_1 \cdot \vec{v}_2 \vec{v}_1 \cdot \vec{v}_2 + 2 (\hat{n} \cdot \vec{S}_1)^2 \vec{v}_1 \cdot \vec{v}_1 \vec{v}_1 \cdot \vec{v}_2 + \\
& 5 \vec{S}_1 \cdot \vec{S}_1 \vec{v}_1 \cdot \vec{v}_1 \vec{v}_1 \cdot \vec{v}_2 + \frac{4}{3} (\vec{S}_1 \cdot \vec{v}_1)^2 \vec{v}_2 \cdot \vec{v}_2 - \frac{2}{3} (\hat{n} \cdot \vec{S}_1)^2 \vec{v}_1 \cdot \vec{v}_1 \vec{v}_2 \cdot \vec{v}_2 - \frac{7}{3} \vec{S}_1 \cdot \vec{S}_1 \vec{v}_1 \cdot \vec{v}_1 \vec{v}_2 \cdot \vec{v}_2 \Big) \Big) m_2 \}
\end{aligned}$$

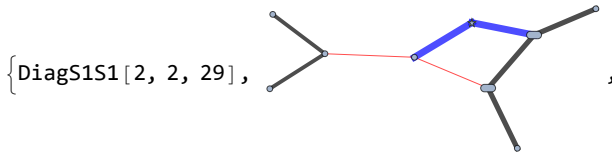

$$\begin{aligned}
& G^2 \left( \frac{1}{r^2} \left( \frac{3}{2} (\hat{n} \times \vec{S}_1 \cdot \vec{v}_1)^2 + 3 \hat{n} \times \vec{S}_1 \cdot \vec{a}_1 \hat{n} \times \vec{S}_1 \cdot \vec{v}_1 + \frac{3}{2} (\hat{n} \times \vec{S}_1 \cdot \vec{a}_1)^2 - (\vec{S}_1 \cdot \vec{v}_1)^2 - (\vec{S}_1 \cdot \vec{a}_1)^2 - \frac{7}{2} (\hat{n} \cdot \vec{v}_1)^2 \vec{S}_1 \cdot \vec{S}_1 + \right. \right. \\
& \frac{7}{2} \hat{n} \cdot \vec{S}_1 \hat{n} \cdot \vec{v}_1 \vec{S}_1 \cdot \vec{a}_1 + \frac{7}{2} \hat{n} \cdot \vec{S}_1 \hat{n} \cdot \vec{v}_1 \vec{S}_1 \cdot \vec{v}_1 - 7 \hat{n} \cdot \vec{a}_1 \hat{n} \cdot \vec{v}_1 \vec{S}_1 \cdot \vec{S}_1 + \frac{7}{2} \hat{n} \cdot \vec{a}_1 \hat{n} \cdot \vec{S}_1 \vec{S}_1 \cdot \vec{a}_1 - \frac{7}{2} (\hat{n} \cdot \vec{a}_1)^2 \vec{S}_1 \cdot \vec{S}_1 + \\
& \left. \vec{a}_1 \cdot \vec{a}_1 \vec{S}_1 \cdot \vec{S}_1 + \frac{7}{2} \hat{n} \cdot \vec{S}_1 \hat{n} \cdot \vec{a}_1 \vec{S}_1 \cdot \vec{v}_1 - 2 \vec{S}_1 \cdot \vec{a}_1 \vec{S}_1 \cdot \vec{v}_1 + 2 \vec{S}_1 \cdot \vec{S}_1 \vec{v}_1 \cdot \vec{a}_1 + \vec{S}_1 \cdot \vec{S}_1 \vec{v}_1 \cdot \vec{v}_1 \right) + \frac{1}{r^3} \\
& \left( 14 \vec{S}_1 \cdot \vec{S}_1 (\hat{n} \cdot \vec{v}_1)^3 - 11 \hat{n} \cdot \vec{S}_1 \vec{S}_1 \cdot \vec{v}_1 (\hat{n} \cdot \vec{v}_1)^2 - 14 \hat{n} \cdot \vec{v}_2 \vec{S}_1 \cdot \vec{S}_1 (\hat{n} \cdot \vec{v}_1)^2 - 3 \hat{n} \cdot \vec{S}_1 \vec{S}_1 \cdot \vec{a}_1 (\hat{n} \cdot \vec{v}_1)^2 + \right.
\end{aligned}$$

$$\begin{aligned}
& 14 \hat{n} \cdot \vec{a}_1 \vec{S}_1 \cdot \vec{S}_1 (\hat{n} \cdot \vec{v}_1)^2 - 3 \hat{n} \cdot \vec{S}_1 \vec{S}_1 \cdot \vec{v}_1 (\hat{n} \cdot \vec{v}_1)^2 - 6 \hat{n} \times \vec{S}_1 \cdot \vec{v}_1 \hat{n} \times \vec{S}_1 \cdot \vec{v}_1 \hat{n} \cdot \vec{v}_1 + 5 \hat{n} \times \vec{S}_1 \cdot \vec{a}_1 \hat{n} \times \vec{S}_1 \cdot \vec{v}_1 \hat{n} \cdot \vec{v}_1 + \\
& 14 \hat{n} \cdot \vec{S}_1 \hat{n} \cdot \vec{v}_2 \vec{S}_1 \cdot \vec{v}_1 \hat{n} \cdot \vec{v}_1 - 14 \hat{n} \cdot \vec{a}_1 \hat{n} \cdot \vec{v}_2 \vec{S}_1 \cdot \vec{S}_1 \hat{n} \cdot \vec{v}_1 + \frac{7}{2} \vec{a}_1 \cdot \vec{v}_2 \vec{S}_1 \cdot \vec{S}_1 \hat{n} \cdot \vec{v}_1 - 11 \hat{n} \cdot \vec{a}_1 \hat{n} \cdot \vec{S}_1 \vec{S}_1 \cdot \vec{v}_1 \hat{n} \cdot \vec{v}_1 + \\
& \frac{11}{2} \vec{S}_1 \cdot \vec{v}_1 \vec{S}_1 \cdot \vec{v}_1 \hat{n} \cdot \vec{v}_1 + \frac{11}{2} \vec{S}_1 \cdot \vec{a}_1 \vec{S}_1 \cdot \vec{v}_1 \hat{n} \cdot \vec{v}_1 - \frac{7}{2} \vec{S}_1 \cdot \vec{v}_1 \vec{S}_1 \cdot \vec{v}_2 \hat{n} \cdot \vec{v}_1 - 8 \vec{S}_1 \cdot \vec{S}_1 \vec{v}_1 \cdot \vec{a}_1 \hat{n} \cdot \vec{v}_1 - \\
& 9 \vec{S}_1 \cdot \vec{S}_1 \vec{v}_1 \cdot \vec{v}_1 \hat{n} \cdot \vec{v}_1 + 7 \vec{S}_1 \cdot \vec{S}_1 \vec{v}_1 \cdot \vec{v}_2 \hat{n} \cdot \vec{v}_1 - \frac{3}{2} \hat{n} \times \vec{S}_1 \cdot \vec{v}_1 \vec{S}_1 \times \vec{v}_1 \cdot \vec{v}_2 - \frac{3}{2} \hat{n} \times \vec{S}_1 \cdot \vec{v}_1 \vec{S}_1 \times \vec{a}_1 \cdot \vec{v}_2 + \\
& 6 \hat{n} \times \vec{S}_1 \cdot \vec{v}_1 \vec{S}_1 \times \vec{v}_1 \cdot \vec{a}_1 - \frac{3}{2} \hat{n} \times \vec{S}_1 \cdot \vec{v}_1 \vec{S}_1 \times \vec{v}_1 \cdot \vec{v}_2 - \frac{3}{2} \hat{n} \times \vec{S}_1 \cdot \vec{a}_1 \vec{S}_1 \times \vec{v}_1 \cdot \vec{v}_2 - 11 (\hat{n} \times \vec{S}_1 \cdot \vec{v}_1)^2 \hat{n} \cdot \vec{a}_1 + \\
& 6 \hat{n} \times \vec{S}_1 \cdot \vec{v}_1 \hat{n} \times \vec{S}_1 \cdot \vec{v}_1 \hat{n} \cdot \vec{v}_2 + 6 \hat{n} \times \vec{S}_1 \cdot \vec{a}_1 \hat{n} \times \vec{S}_1 \cdot \vec{v}_1 \hat{n} \cdot \vec{v}_2 + 14 \hat{n} \cdot \vec{a}_1 \hat{n} \cdot \vec{S}_1 \hat{n} \cdot \vec{v}_2 \vec{S}_1 \cdot \vec{v}_1 - 2 \hat{n} \cdot \vec{v}_2 \vec{S}_1 \cdot \vec{v}_1 \vec{S}_1 \cdot \vec{v}_1 - \\
& \frac{7}{2} \hat{n} \cdot \vec{S}_1 \vec{a}_1 \cdot \vec{v}_2 \vec{S}_1 \cdot \vec{v}_1 - 2 \hat{n} \cdot \vec{v}_2 \vec{S}_1 \cdot \vec{a}_1 \vec{S}_1 \cdot \vec{v}_1 - \frac{7}{2} \hat{n} \cdot \vec{a}_1 \vec{S}_1 \cdot \vec{v}_1 \vec{S}_1 \cdot \vec{v}_2 + 2 \hat{n} \cdot \vec{v}_2 \vec{S}_1 \cdot \vec{S}_1 \vec{v}_1 \cdot \vec{a}_1 + \\
& \frac{5}{2} \hat{n} \cdot \vec{S}_1 \vec{S}_1 \cdot \vec{v}_1 \vec{v}_1 \cdot \vec{a}_1 + \frac{5}{2} \hat{n} \cdot \vec{S}_1 \vec{S}_1 \cdot \vec{v}_1 \vec{v}_1 \cdot \vec{v}_1 + 2 \hat{n} \cdot \vec{v}_2 \vec{S}_1 \cdot \vec{S}_1 \vec{v}_1 \cdot \vec{v}_1 + \hat{n} \cdot \vec{S}_1 \vec{S}_1 \cdot \vec{a}_1 \vec{v}_1 \cdot \vec{v}_1 - \\
& \hat{n} \cdot \vec{a}_1 \vec{S}_1 \cdot \vec{S}_1 \vec{v}_1 \cdot \vec{v}_1 + \hat{n} \cdot \vec{S}_1 \vec{S}_1 \cdot \vec{v}_1 \vec{v}_1 \cdot \vec{v}_1 - \frac{7}{2} \hat{n} \cdot \vec{S}_1 \vec{S}_1 \cdot \vec{v}_1 \vec{v}_1 \cdot \vec{v}_2 + \frac{7}{2} \hat{n} \cdot \vec{a}_1 \vec{S}_1 \cdot \vec{S}_1 \vec{v}_1 \cdot \vec{v}_2 \Big) + \frac{1}{r^4} \\
& \left( -\frac{39}{4} \vec{S}_1 \cdot \vec{S}_1 (\hat{n} \cdot \vec{v}_1)^4 + 18 \hat{n} \cdot \vec{v}_2 \vec{S}_1 \cdot \vec{S}_1 (\hat{n} \cdot \vec{v}_1)^3 + \frac{39}{4} \hat{n} \cdot \vec{S}_1 \vec{S}_1 \cdot \vec{v}_1 (\hat{n} \cdot \vec{v}_1)^3 - \frac{171}{4} (\hat{n} \times \vec{S}_1 \cdot \vec{v}_1)^2 (\hat{n} \cdot \vec{v}_1)^2 - \right. \\
& 12 (\vec{S}_1 \cdot \vec{v}_1)^2 (\hat{n} \cdot \vec{v}_1)^2 - 18 \hat{n} \cdot \vec{S}_1 \hat{n} \cdot \vec{v}_2 \vec{S}_1 \cdot \vec{v}_1 (\hat{n} \cdot \vec{v}_1)^2 + 3 \vec{S}_1 \cdot \vec{v}_1 \vec{S}_1 \cdot \vec{v}_2 (\hat{n} \cdot \vec{v}_1)^2 + \frac{75}{4} \vec{S}_1 \cdot \vec{S}_1 \vec{v}_1 \cdot \vec{v}_1 (\hat{n} \cdot \vec{v}_1)^2 - \\
& 9 \vec{S}_1 \cdot \vec{S}_1 \vec{v}_1 \cdot \vec{v}_2 (\hat{n} \cdot \vec{v}_1)^2 + 16 \hat{n} \cdot \vec{v}_2 (\vec{S}_1 \cdot \vec{v}_1)^2 \hat{n} \cdot \vec{v}_1 - 20 \hat{n} \times \vec{S}_1 \cdot \vec{v}_1 \vec{S}_1 \times \vec{v}_1 \cdot \vec{v}_2 \hat{n} \cdot \vec{v}_1 + 60 (\hat{n} \times \vec{S}_1 \cdot \vec{v}_1)^2 \\
& \hat{n} \cdot \vec{v}_2 \hat{n} \cdot \vec{v}_1 - 20 \hat{n} \cdot \vec{v}_2 \vec{S}_1 \cdot \vec{S}_1 \vec{v}_1 \cdot \vec{v}_1 \hat{n} \cdot \vec{v}_1 - \frac{27}{4} \hat{n} \cdot \vec{S}_1 \vec{S}_1 \cdot \vec{v}_1 \vec{v}_1 \cdot \vec{v}_1 \hat{n} \cdot \vec{v}_1 + 6 \hat{n} \cdot \vec{S}_1 \vec{S}_1 \cdot \vec{v}_1 \vec{v}_1 \cdot \vec{v}_2 \hat{n} \cdot \vec{v}_1 - \\
& 3 \vec{S}_1 \cdot \vec{S}_1 (\vec{v}_1 \cdot \vec{v}_1)^2 + \frac{21}{4} (\hat{n} \times \vec{S}_1 \cdot \vec{v}_1)^2 \vec{v}_1 \cdot \vec{v}_1 + 3 (\vec{S}_1 \cdot \vec{v}_1)^2 \vec{v}_1 \cdot \vec{v}_1 + 4 \hat{n} \cdot \vec{S}_1 \hat{n} \cdot \vec{v}_2 \vec{S}_1 \cdot \vec{v}_1 \vec{v}_1 \cdot \vec{v}_1 - \\
& \left. \vec{S}_1 \cdot \vec{v}_1 \vec{S}_1 \cdot \vec{v}_2 \vec{v}_1 \cdot \vec{v}_1 - 10 (\hat{n} \times \vec{S}_1 \cdot \vec{v}_1)^2 \vec{v}_1 \cdot \vec{v}_2 - 4 (\vec{S}_1 \cdot \vec{v}_1)^2 \vec{v}_1 \cdot \vec{v}_2 + 5 \vec{S}_1 \cdot \vec{S}_1 \vec{v}_1 \cdot \vec{v}_1 \vec{v}_1 \cdot \vec{v}_2 \right) \Big) m_2 \Big\}
\end{aligned}$$

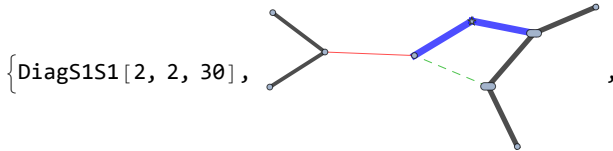

$$\begin{aligned}
& G^2 \left( \frac{1}{r} \left( \frac{2}{3} \hat{n} \cdot \vec{S}_1 \hat{n} \cdot \vec{a}_1 \hat{n} \cdot \vec{S}_1 - \frac{1}{3} \vec{S}_1 \cdot \vec{a}_1 \hat{n} \cdot \vec{S}_1 + \frac{2}{3} \hat{n} \cdot \vec{S}_1 \hat{n} \cdot \vec{S}_1 \hat{n} \cdot \vec{v}_1 - \right. \right. \\
& \left. \frac{7}{3} \hat{n} \cdot \vec{v}_1 \vec{S}_1 \cdot \vec{S}_1 + \frac{2}{3} \hat{n} \cdot \vec{S}_1 \vec{S}_1 \cdot \vec{v}_1 - \frac{1}{3} \hat{n} \cdot \vec{S}_1 \vec{S}_1 \cdot \vec{v}_1 - \frac{7}{3} \hat{n} \cdot \vec{a}_1 \vec{S}_1 \cdot \vec{S}_1 + \frac{2}{3} \hat{n} \cdot \vec{S}_1 \vec{S}_1 \cdot \vec{a}_1 \right) + \frac{1}{r^2} \\
& \left( -3 (\hat{n} \times \vec{S}_1 \cdot \vec{v}_1)^2 - \frac{3}{2} (\hat{n} \times \vec{S}_1 \cdot \vec{a}_1)^2 - 2 (\hat{n} \cdot \vec{a}_1)^2 (\hat{n} \cdot \vec{S}_1)^2 + 2 \hat{n} \cdot \vec{a}_1 \hat{n} \cdot \vec{a}_2 (\hat{n} \cdot \vec{S}_1)^2 - 4 (\hat{n} \cdot \vec{S}_1)^2 (\hat{n} \cdot \vec{v}_1)^2 - \right. \\
& \frac{2}{3} \hat{n} \cdot \vec{S}_1 \hat{n} \cdot \vec{S}_1 (\hat{n} \cdot \vec{v}_1)^2 - \frac{9}{2} \hat{n} \times \vec{S}_1 \cdot \vec{a}_1 \hat{n} \times \vec{S}_1 \cdot \vec{v}_1 + \frac{3}{2} \hat{n} \times \vec{S}_1 \cdot \vec{v}_1 \hat{n} \times \vec{S}_1 \cdot \vec{v}_1 - 6 \hat{n} \cdot \vec{S}_1 \hat{n} \cdot \vec{a}_1 \hat{n} \cdot \vec{S}_1 \hat{n} \cdot \vec{v}_1 + \\
& 2 \hat{n} \cdot \vec{S}_1 \hat{n} \cdot \vec{a}_2 \hat{n} \cdot \vec{S}_1 \hat{n} \cdot \vec{v}_1 + \frac{14}{3} \hat{n} \cdot \vec{S}_1 \hat{n} \cdot \vec{a}_1 \hat{n} \cdot \vec{S}_1 \hat{n} \cdot \vec{v}_2 + \frac{14}{3} (\hat{n} \cdot \vec{S}_1)^2 \hat{n} \cdot \vec{v}_1 \hat{n} \cdot \vec{v}_2 + 9 (\hat{n} \cdot \vec{v}_1)^2 \vec{S}_1 \cdot \vec{S}_1 - \\
& \frac{29}{3} \hat{n} \cdot \vec{v}_1 \hat{n} \cdot \vec{v}_2 \vec{S}_1 \cdot \vec{S}_1 + 2 \hat{n} \cdot \vec{S}_1 \hat{n} \cdot \vec{v}_1 \vec{S}_1 \cdot \vec{a}_1 + \frac{1}{3} \hat{n} \cdot \vec{S}_1 \hat{n} \cdot \vec{v}_2 \vec{S}_1 \cdot \vec{a}_1 - \frac{1}{2} \hat{n} \cdot \vec{S}_1 \hat{n} \cdot \vec{v}_1 \vec{S}_1 \cdot \vec{a}_2 - \\
& 3 \hat{n} \cdot \vec{a}_1 \hat{n} \cdot \vec{S}_1 \vec{S}_1 \cdot \vec{v}_1 + \hat{n} \cdot \vec{a}_2 \hat{n} \cdot \vec{S}_1 \vec{S}_1 \cdot \vec{v}_1 - \hat{n} \cdot \vec{S}_1 \hat{n} \cdot \vec{v}_1 \vec{S}_1 \cdot \vec{v}_1 + \frac{8}{3} \hat{n} \cdot \vec{S}_1 \hat{n} \cdot \vec{v}_2 \vec{S}_1 \cdot \vec{v}_1 - \frac{7}{6} \hat{n} \cdot \vec{a}_1 \hat{n} \cdot \vec{S}_1 \vec{S}_1 \cdot \vec{v}_2 - \\
& \frac{7}{3} \hat{n} \cdot \vec{S}_1 \hat{n} \cdot \vec{v}_1 \vec{S}_1 \cdot \vec{v}_2 - \frac{4}{3} \vec{S}_1 \cdot \vec{v}_1 \vec{S}_1 \cdot \vec{v}_2 + \frac{11}{6} \hat{n} \cdot \vec{S}_1 \hat{n} \cdot \vec{v}_1 \vec{S}_1 \cdot \vec{v}_1 + \frac{1}{2} (\hat{n} \cdot \vec{S}_1)^2 \vec{a}_1 \cdot \vec{a}_1 - \frac{1}{2} (\hat{n} \cdot \vec{S}_1)^2 \vec{a}_1 \cdot \vec{a}_2 - \\
& \left. \frac{7}{6} \hat{n} \cdot \vec{S}_1 \hat{n} \cdot \vec{S}_1 \vec{a}_1 \cdot \vec{v}_2 + \frac{27}{2} \hat{n} \cdot \vec{a}_1 \hat{n} \cdot \vec{v}_1 \vec{S}_1 \cdot \vec{S}_1 - 5 \hat{n} \cdot \vec{a}_2 \hat{n} \cdot \vec{v}_1 \vec{S}_1 \cdot \vec{S}_1 - \frac{29}{3} \hat{n} \cdot \vec{a}_1 \hat{n} \cdot \vec{v}_2 \vec{S}_1 \cdot \vec{S}_1 + \right. \\
& \left. \frac{1}{3} \hat{n} \cdot \vec{S}_1 \hat{n} \cdot \vec{v}_1 \vec{S}_1 \cdot \vec{v}_1 \right) \Big)
\end{aligned}$$



$$\{\text{DiagS1S1}[2, 2, 31],$$

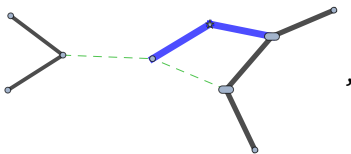



$$\begin{aligned}
& \frac{1}{r^4} \left( \frac{63}{4} \hat{n} \cdot \vec{v}_2 \vec{S}_1 \cdot \vec{S}_1 (\hat{n} \cdot \vec{v}_1)^3 - \frac{9}{2} \hat{n} \cdot \vec{S}_1 \vec{S}_1 \cdot \vec{v}_2 (\hat{n} \cdot \vec{v}_1)^3 - 2 (\vec{S}_1 \cdot \vec{v}_2)^2 (\hat{n} \cdot \vec{v}_1)^2 + \right. \\
& 151 \hat{n} \times \vec{S}_1 \cdot \vec{v}_1 \hat{n} \times \vec{S}_1 \cdot \vec{v}_2 (\hat{n} \cdot \vec{v}_1)^2 - 30 (\hat{n} \cdot \vec{v}_2)^2 \vec{S}_1 \cdot \vec{S}_1 (\hat{n} \cdot \vec{v}_1)^2 - \frac{45}{4} \hat{n} \cdot \vec{S}_1 \hat{n} \cdot \vec{v}_2 \vec{S}_1 \cdot \vec{v}_1 (\hat{n} \cdot \vec{v}_1)^2 + \\
& 12 \hat{n} \cdot \vec{S}_1 \hat{n} \cdot \vec{v}_2 \vec{S}_1 \cdot \vec{v}_2 (\hat{n} \cdot \vec{v}_1)^2 + \frac{45}{4} \vec{S}_1 \cdot \vec{v}_1 \vec{S}_1 \cdot \vec{v}_2 (\hat{n} \cdot \vec{v}_1)^2 + \frac{33}{4} (\hat{n} \cdot \vec{S}_1)^2 \vec{v}_1 \cdot \vec{v}_2 (\hat{n} \cdot \vec{v}_1)^2 - \\
& \frac{27}{2} \vec{S}_1 \cdot \vec{S}_1 \vec{v}_1 \cdot \vec{v}_2 (\hat{n} \cdot \vec{v}_1)^2 + 5 \vec{S}_1 \cdot \vec{S}_1 \vec{v}_2 \cdot \vec{v}_2 (\hat{n} \cdot \vec{v}_1)^2 + 4 \hat{n} \cdot \vec{v}_2 (\vec{S}_1 \cdot \vec{v}_1)^2 \hat{n} \cdot \vec{v}_1 + \\
& 14 \hat{n} \times \vec{S}_1 \cdot \vec{v}_1 \vec{S}_1 \times \vec{v}_1 \cdot \vec{v}_2 \hat{n} \cdot \vec{v}_1 + 13 \hat{n} \times \vec{S}_1 \cdot \vec{v}_2 \vec{S}_1 \times \vec{v}_1 \cdot \vec{v}_2 \hat{n} \cdot \vec{v}_1 - \frac{3}{2} (\hat{n} \times \vec{S}_1 \cdot \vec{v}_1)^2 \hat{n} \cdot \vec{v}_2 \hat{n} \cdot \vec{v}_1 - \\
& 78 \hat{n} \times \vec{S}_1 \cdot \vec{v}_1 \hat{n} \times \vec{S}_1 \cdot \vec{v}_2 \hat{n} \cdot \vec{v}_2 \hat{n} \cdot \vec{v}_1 + 18 \hat{n} \cdot \vec{S}_1 (\hat{n} \cdot \vec{v}_2)^2 \vec{S}_1 \cdot \vec{v}_1 \hat{n} \cdot \vec{v}_1 - 19 \hat{n} \cdot \vec{v}_2 \vec{S}_1 \cdot \vec{v}_1 \vec{S}_1 \cdot \vec{v}_2 \hat{n} \cdot \vec{v}_1 - \\
& \frac{3}{2} (\hat{n} \cdot \vec{S}_1)^2 \hat{n} \cdot \vec{v}_2 \vec{v}_1 \cdot \vec{v}_1 \hat{n} \cdot \vec{v}_1 - \frac{47}{4} \hat{n} \cdot \vec{v}_2 \vec{S}_1 \cdot \vec{S}_1 \vec{v}_1 \cdot \vec{v}_1 \hat{n} \cdot \vec{v}_1 + \frac{7}{2} \hat{n} \cdot \vec{S}_1 \vec{S}_1 \cdot \vec{v}_2 \vec{v}_1 \cdot \vec{v}_1 \hat{n} \cdot \vec{v}_1 - \\
& 18 (\hat{n} \cdot \vec{S}_1)^2 \hat{n} \cdot \vec{v}_2 \vec{v}_1 \cdot \vec{v}_2 \hat{n} \cdot \vec{v}_1 + 30 \hat{n} \cdot \vec{v}_2 \vec{S}_1 \cdot \vec{S}_1 \vec{v}_1 \cdot \vec{v}_2 \hat{n} \cdot \vec{v}_1 - \frac{9}{2} \hat{n} \cdot \vec{S}_1 \vec{S}_1 \cdot \vec{v}_1 \vec{v}_1 \cdot \vec{v}_2 \hat{n} \cdot \vec{v}_1 + \\
& 2 \hat{n} \cdot \vec{S}_1 \vec{S}_1 \cdot \vec{v}_2 \vec{v}_1 \cdot \vec{v}_2 \hat{n} \cdot \vec{v}_1 - 3 \hat{n} \cdot \vec{S}_1 \vec{S}_1 \cdot \vec{v}_1 \vec{v}_2 \cdot \vec{v}_2 \hat{n} \cdot \vec{v}_1 + 2 (\vec{S}_1 \times \vec{v}_1 \cdot \vec{v}_2)^2 + 6 (\hat{n} \times \vec{S}_1 \cdot \vec{v}_1)^2 (\hat{n} \cdot \vec{v}_2)^2 - \\
& 4 (\hat{n} \cdot \vec{v}_2)^2 (\vec{S}_1 \cdot \vec{v}_1)^2 + 3 (\hat{n} \cdot \vec{S}_1)^2 (\vec{v}_1 \cdot \vec{v}_2)^2 - 5 \vec{S}_1 \cdot \vec{S}_1 (\vec{v}_1 \cdot \vec{v}_2)^2 - 10 \hat{n} \times \vec{S}_1 \cdot \vec{v}_1 \vec{S}_1 \times \vec{v}_1 \cdot \vec{v}_2 \hat{n} \cdot \vec{v}_2 + \\
& 6 (\hat{n} \cdot \vec{S}_1)^2 (\hat{n} \cdot \vec{v}_2)^2 \vec{v}_1 \cdot \vec{v}_1 + (\vec{S}_1 \cdot \vec{v}_2)^2 \vec{v}_1 \cdot \vec{v}_1 - 6 \hat{n} \times \vec{S}_1 \cdot \vec{v}_1 \hat{n} \times \vec{S}_1 \cdot \vec{v}_2 \vec{v}_1 \cdot \vec{v}_1 + \\
& 8 (\hat{n} \cdot \vec{v}_2)^2 \vec{S}_1 \cdot \vec{S}_1 \vec{v}_1 \cdot \vec{v}_1 + \frac{19}{4} \hat{n} \cdot \vec{S}_1 \hat{n} \cdot \vec{v}_2 \vec{S}_1 \cdot \vec{v}_1 \vec{v}_1 \cdot \vec{v}_1 - 6 \hat{n} \cdot \vec{S}_1 \hat{n} \cdot \vec{v}_2 \vec{S}_1 \cdot \vec{v}_2 \vec{v}_1 \cdot \vec{v}_1 - \\
& \frac{13}{4} \vec{S}_1 \cdot \vec{v}_1 \vec{S}_1 \cdot \vec{v}_2 \vec{v}_1 \cdot \vec{v}_1 - \frac{1}{2} (\hat{n} \times \vec{S}_1 \cdot \vec{v}_1)^2 \vec{v}_1 \cdot \vec{v}_2 + \frac{1}{2} (\vec{S}_1 \cdot \vec{v}_1)^2 \vec{v}_1 \cdot \vec{v}_2 + 13 \hat{n} \times \vec{S}_1 \cdot \vec{v}_1 \hat{n} \times \vec{S}_1 \cdot \vec{v}_2 \vec{v}_1 \cdot \vec{v}_2 + \\
& \hat{n} \cdot \vec{S}_1 \hat{n} \cdot \vec{v}_2 \vec{S}_1 \cdot \vec{v}_1 \vec{v}_1 \cdot \vec{v}_2 + 3 \vec{S}_1 \cdot \vec{v}_1 \vec{S}_1 \cdot \vec{v}_2 \vec{v}_1 \cdot \vec{v}_2 - \frac{5}{4} (\hat{n} \cdot \vec{S}_1)^2 \vec{v}_1 \cdot \vec{v}_1 \vec{v}_1 \cdot \vec{v}_2 + \frac{7}{2} \vec{S}_1 \cdot \vec{S}_1 \vec{v}_1 \cdot \vec{v}_1 \vec{v}_1 \cdot \vec{v}_2 - \\
& \left. (\hat{n} \times \vec{S}_1 \cdot \vec{v}_1)^2 \vec{v}_2 \cdot \vec{v}_2 + (\vec{S}_1 \cdot \vec{v}_1)^2 \vec{v}_2 \cdot \vec{v}_2 - (\hat{n} \cdot \vec{S}_1)^2 \vec{v}_1 \cdot \vec{v}_1 \vec{v}_2 \cdot \vec{v}_2 - 2 \vec{S}_1 \cdot \vec{S}_1 \vec{v}_1 \cdot \vec{v}_1 \vec{v}_2 \cdot \vec{v}_2 \right) m_2 \}
\end{aligned}$$

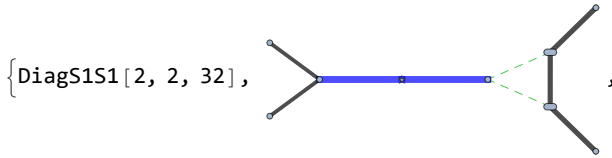

$$\begin{aligned}
& G^2 \left( \frac{1}{r^2} \left( -\frac{1}{2} \hat{n} \times \vec{S}_1 \cdot \vec{v}_2 \hat{n} \times \vec{S}_1 \cdot \vec{a}_2 - \frac{1}{2} \hat{n} \times \vec{S}_1 \cdot \vec{a}_2 \hat{n} \times \vec{S}_1 \cdot \vec{v}_2 + \frac{1}{2} \hat{n} \cdot \vec{S}_1 \hat{n} \cdot \vec{a}_2 \hat{n} \cdot \vec{S}_1 \cdot \vec{v}_2 + \right. \right. \\
& \frac{1}{2} \hat{n} \cdot \vec{S}_1 \hat{n} \cdot \vec{v}_2 \vec{S}_1 \cdot \vec{a}_2 + \frac{1}{2} \hat{n} \cdot \vec{a}_2 \hat{n} \cdot \vec{S}_1 \vec{S}_1 \cdot \vec{v}_2 - \frac{3}{2} \hat{n} \cdot \vec{a}_2 \hat{n} \cdot \vec{v}_2 \vec{S}_1 \cdot \vec{S}_1 + \frac{1}{2} \hat{n} \cdot \vec{S}_1 \hat{n} \cdot \vec{v}_2 \vec{S}_1 \cdot \vec{a}_2 - \\
& \left. \frac{1}{2} \vec{S}_1 \cdot \vec{v}_2 \vec{S}_1 \cdot \vec{a}_2 + \frac{1}{2} \hat{n} \cdot \vec{S}_1 \hat{n} \cdot \vec{a}_2 \vec{S}_1 \cdot \vec{v}_2 - \frac{1}{2} \vec{S}_1 \cdot \vec{a}_2 \vec{S}_1 \cdot \vec{v}_2 - \frac{3}{2} \hat{n} \cdot \vec{S}_1 \hat{n} \cdot \vec{S}_1 \vec{v}_2 \cdot \vec{a}_2 + \frac{3}{2} \vec{S}_1 \cdot \vec{S}_1 \vec{v}_2 \cdot \vec{a}_2 \right) + \\
& \frac{1}{r^3} \left( \frac{3}{2} \hat{n} \cdot \vec{S}_1 \hat{n} \cdot \vec{S}_1 (\hat{n} \cdot \vec{v}_2)^3 - 3 \vec{S}_1 \cdot \vec{S}_1 (\hat{n} \cdot \vec{v}_2)^3 + \frac{7}{4} \hat{n} \cdot \vec{S}_1 \vec{S}_1 \cdot \vec{v}_2 (\hat{n} \cdot \vec{v}_2)^2 + \frac{7}{4} \hat{n} \cdot \vec{S}_1 \vec{S}_1 \cdot \vec{v}_2 (\hat{n} \cdot \vec{v}_2)^2 - \right. \\
& 2 \hat{n} \times \vec{S}_1 \cdot \vec{v}_2 \hat{n} \times \vec{S}_1 \cdot \vec{v}_2 \hat{n} \cdot \vec{v}_2 - \frac{3}{2} \hat{n} \cdot \vec{a}_2 (\hat{n} \cdot \vec{S}_1)^2 \hat{n} \cdot \vec{v}_1 \hat{n} \cdot \vec{v}_2 - 2 \hat{n} \cdot \vec{S}_1 \hat{n} \cdot \vec{v}_1 \vec{S}_1 \cdot \vec{a}_2 \hat{n} \cdot \vec{v}_2 + \\
& 3 \hat{n} \cdot \vec{a}_2 \hat{n} \cdot \vec{v}_1 \vec{S}_1 \cdot \vec{S}_1 \hat{n} \cdot \vec{v}_2 + \frac{1}{2} \hat{n} \cdot \vec{a}_2 \hat{n} \cdot \vec{S}_1 \vec{S}_1 \cdot \vec{v}_1 \hat{n} \cdot \vec{v}_2 + \frac{1}{2} \vec{S}_1 \cdot \vec{a}_2 \vec{S}_1 \cdot \vec{v}_1 \hat{n} \cdot \vec{v}_2 - \\
& 2 \vec{S}_1 \cdot \vec{v}_2 \vec{S}_1 \cdot \vec{v}_2 \hat{n} \cdot \vec{v}_2 + \frac{1}{4} (\hat{n} \cdot \vec{S}_1)^2 \vec{v}_1 \cdot \vec{a}_2 \hat{n} \cdot \vec{v}_2 - \frac{3}{4} \vec{S}_1 \cdot \vec{S}_1 \vec{v}_1 \cdot \vec{a}_2 \hat{n} \cdot \vec{v}_2 - \frac{7}{2} \hat{n} \cdot \vec{S}_1 \hat{n} \cdot \vec{S}_1 \vec{v}_2 \cdot \vec{v}_2 \hat{n} \cdot \vec{v}_2 + \\
& 3 \vec{S}_1 \cdot \vec{S}_1 \vec{v}_2 \cdot \vec{v}_2 \hat{n} \cdot \vec{v}_2 + \frac{1}{2} \hat{n} \times \vec{S}_1 \cdot \vec{v}_2 \vec{S}_1 \times \vec{v}_1 \cdot \vec{a}_2 + \frac{1}{2} \hat{n} \times \vec{S}_1 \cdot \vec{a}_2 \vec{S}_1 \times \vec{v}_1 \cdot \vec{v}_2 + 2 \hat{n} \times \vec{S}_1 \cdot \vec{a}_2 \hat{n} \times \vec{S}_1 \cdot \vec{v}_2 \hat{n} \cdot \vec{v}_1 - \\
& 2 \hat{n} \cdot \vec{a}_2 \hat{n} \cdot \vec{S}_1 \hat{n} \cdot \vec{v}_1 \vec{S}_1 \cdot \vec{v}_2 + \hat{n} \cdot \vec{v}_1 \vec{S}_1 \cdot \vec{a}_2 \vec{S}_1 \cdot \vec{v}_2 + \frac{1}{2} \hat{n} \cdot \vec{a}_2 \vec{S}_1 \cdot \vec{v}_1 \vec{S}_1 \cdot \vec{v}_2 + \frac{1}{2} \hat{n} \cdot \vec{S}_1 \vec{S}_1 \cdot \vec{v}_2 \vec{v}_1 \cdot \vec{a}_2 + \\
& \left. \frac{1}{4} \hat{n} \cdot \vec{a}_2 (\hat{n} \cdot \vec{S}_1)^2 \vec{v}_1 \cdot \vec{v}_2 + \frac{1}{2} \hat{n} \cdot \vec{S}_1 \vec{S}_1 \cdot \vec{a}_2 \vec{v}_1 \cdot \vec{v}_2 - \frac{3}{4} \hat{n} \cdot \vec{a}_2 \vec{S}_1 \cdot \vec{S}_1 \vec{v}_1 \cdot \vec{v}_2 + 3 (\hat{n} \cdot \vec{S}_1)^2 \hat{n} \cdot \vec{v}_1 \vec{v}_2 \cdot \vec{a}_2 - \right.
\end{aligned}$$

$$\begin{aligned} & \frac{3}{2} \hat{n} \cdot \vec{v}_1 \vec{S}_1 \cdot \vec{S}_1 \vec{v}_2 \cdot \vec{a}_2 - \frac{3}{2} \hat{n} \cdot \vec{S}_1 \vec{S}_1 \cdot \vec{v}_1 \vec{v}_2 \cdot \vec{a}_2 + \frac{1}{4} \hat{n} \cdot \vec{S}_1 \vec{S}_1 \cdot \vec{v}_2 \vec{v}_2 \cdot \vec{v}_2 + \frac{1}{4} \hat{n} \cdot \vec{S}_1 \vec{S}_1 \cdot \vec{v}_2 \vec{v}_2 \cdot \vec{v}_2 \Big) + \\ & \frac{1}{\rho^4} \left( -6 \left( \hat{n} \cdot \vec{S}_1 \right)^2 \hat{n} \cdot \vec{v}_1 \left( \hat{n} \cdot \vec{v}_2 \right)^3 + 9 \hat{n} \cdot \vec{v}_1 \vec{S}_1 \cdot \vec{S}_1 \left( \hat{n} \cdot \vec{v}_2 \right)^3 + \frac{3}{2} \hat{n} \cdot \vec{S}_1 \vec{S}_1 \cdot \vec{v}_1 \left( \hat{n} \cdot \vec{v}_2 \right)^3 - \right. \\ & \frac{21}{2} \hat{n} \cdot \vec{S}_1 \hat{n} \cdot \vec{v}_1 \vec{S}_1 \cdot \vec{v}_2 \left( \hat{n} \cdot \vec{v}_2 \right)^2 + \frac{7}{4} \vec{S}_1 \cdot \vec{v}_1 \vec{S}_1 \cdot \vec{v}_2 \left( \hat{n} \cdot \vec{v}_2 \right)^2 + \frac{9}{4} \left( \hat{n} \cdot \vec{S}_1 \right)^2 \vec{v}_1 \cdot \vec{v}_2 \left( \hat{n} \cdot \vec{v}_2 \right)^2 - \\ & \frac{9}{2} \vec{S}_1 \cdot \vec{S}_1 \vec{v}_1 \cdot \vec{v}_2 \left( \hat{n} \cdot \vec{v}_2 \right)^2 + 4 \hat{n} \cdot \vec{v}_1 \left( \vec{S}_1 \cdot \vec{v}_2 \right)^2 \hat{n} \cdot \vec{v}_2 + 2 \hat{n} \times \vec{S}_1 \cdot \vec{v}_2 \vec{S}_1 \times \vec{v}_1 \cdot \vec{v}_2 \hat{n} \cdot \vec{v}_2 + \\ & 6 \left( \hat{n} \times \vec{S}_1 \cdot \vec{v}_2 \right)^2 \hat{n} \cdot \vec{v}_1 \hat{n} \cdot \vec{v}_2 + \frac{7}{2} \hat{n} \cdot \vec{S}_1 \vec{S}_1 \cdot \vec{v}_2 \vec{v}_1 \cdot \vec{v}_2 \hat{n} \cdot \vec{v}_2 + \frac{21}{2} \left( \hat{n} \cdot \vec{S}_1 \right)^2 \hat{n} \cdot \vec{v}_1 \vec{v}_2 \cdot \vec{v}_2 \hat{n} \cdot \vec{v}_2 - \\ & 6 \hat{n} \cdot \vec{v}_1 \vec{S}_1 \cdot \vec{S}_1 \vec{v}_2 \cdot \vec{v}_2 \hat{n} \cdot \vec{v}_2 - \frac{7}{2} \hat{n} \cdot \vec{S}_1 \vec{S}_1 \cdot \vec{v}_1 \vec{v}_2 \cdot \vec{v}_2 \hat{n} \cdot \vec{v}_2 - \left( \hat{n} \times \vec{S}_1 \cdot \vec{v}_2 \right)^2 \vec{v}_1 \cdot \vec{v}_2 - \left( \vec{S}_1 \cdot \vec{v}_2 \right)^2 \vec{v}_1 \cdot \vec{v}_2 - \\ & \left. \hat{n} \cdot \vec{S}_1 \hat{n} \cdot \vec{v}_1 \vec{S}_1 \cdot \vec{v}_2 \vec{v}_2 \cdot \vec{v}_2 + \frac{1}{4} \vec{S}_1 \cdot \vec{v}_1 \vec{S}_1 \cdot \vec{v}_2 \vec{v}_2 \cdot \vec{v}_2 - \frac{7}{4} \left( \hat{n} \cdot \vec{S}_1 \right)^2 \vec{v}_1 \cdot \vec{v}_2 \vec{v}_2 \cdot \vec{v}_2 + \frac{3}{2} \vec{S}_1 \cdot \vec{S}_1 \vec{v}_1 \cdot \vec{v}_2 \vec{v}_2 \cdot \vec{v}_2 \right) \Big) m_2 \} \end{aligned}$$

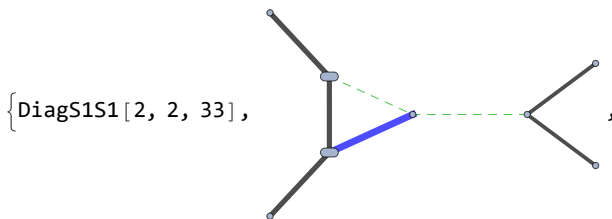

$$G^2 \left( \frac{\hat{n} \times \vec{S_1} \cdot \vec{v_1} \hat{n} \times \vec{S_1} \cdot \vec{a_2} + \vec{S_1} \cdot \vec{a_2} \vec{S_1} \cdot \vec{v_1} - \hat{n} \cdot \vec{S_1} \hat{n} \cdot \vec{S_1} \vec{v_1} \cdot \vec{a_2} - 2 \vec{S_1} \cdot \vec{S_1} \vec{v_1} \cdot \vec{a_2}}{r^2} + \frac{1}{r^3} \right. \\ \left. \left( 2 \hat{n} \cdot \vec{v_1} \vec{v_1} \cdot \vec{a_2} \left( \hat{n} \cdot \vec{S_1} \right)^2 + \vec{a_1} \cdot \vec{v_2} \vec{S_1} \cdot \vec{v_1} \hat{n} \cdot \vec{S_1} - \vec{S_1} \cdot \vec{v_1} \vec{v_1} \cdot \vec{a_2} \hat{n} \cdot \vec{S_1} - 4 \hat{n} \cdot \vec{S_1} \hat{n} \cdot \vec{v_2} \vec{v_1} \cdot \vec{v_2} \hat{n} \cdot \vec{S_1} + \vec{S_1} \cdot \vec{v_2} \vec{v_1} \cdot \vec{v_2} \right. \right. \\ \left. \left. \hat{n} \cdot \vec{S_1} + 4 \vec{S_1} \cdot \vec{a_1} \vec{v_1} \cdot \vec{v_2} \hat{n} \cdot \vec{S_1} - \frac{17}{2} \hat{n} \times \vec{S_1} \cdot \vec{v_1} \vec{S_1} \times \vec{v_1} \cdot \vec{v_2} - \hat{n} \times \vec{S_1} \cdot \vec{v_2} \vec{S_1} \times \vec{v_1} \cdot \vec{v_2} - 12 \hat{n} \times \vec{S_1} \cdot \vec{v_1} \vec{S_1} \times \vec{a_1} \cdot \vec{v_2} - \right. \right. \\ \left. \left. 10 \hat{n} \times \vec{S_1} \cdot \vec{v_2} \vec{S_1} \times \vec{v_1} \cdot \vec{a_1} - \hat{n} \times \vec{S_1} \cdot \vec{v_1} \vec{S_1} \times \vec{v_1} \cdot \vec{a_2} - \hat{n} \times \vec{S_1} \cdot \vec{a_1} \vec{S_1} \times \vec{v_1} \cdot \vec{v_2} - 24 \hat{n} \times \vec{S_1} \cdot \vec{v_1} \hat{n} \times \vec{S_1} \cdot \vec{v_2} \hat{n} \cdot \vec{a_1} - \right. \right. \\ \left. \left. 2 \hat{n} \times \vec{S_1} \cdot \vec{a_2} \hat{n} \times \vec{S_1} \cdot \vec{v_1} \hat{n} \cdot \vec{v_1} - 36 \hat{n} \times \vec{S_1} \cdot \vec{v_1} \hat{n} \times \vec{S_1} \cdot \vec{v_2} \hat{n} \cdot \vec{v_1} - 48 \hat{n} \times \vec{S_1} \cdot \vec{a_1} \hat{n} \times \vec{S_1} \cdot \vec{v_2} \hat{n} \cdot \vec{v_1} + \right. \right. \\ \left. \left. 4 \hat{n} \times \vec{S_1} \cdot \vec{v_1} \hat{n} \times \vec{S_1} \cdot \vec{v_2} \hat{n} \cdot \vec{v_2} + 11 \hat{n} \cdot \vec{v_1} \vec{a_1} \cdot \vec{v_2} \vec{S_1} \cdot \vec{S_1} + 6 \hat{n} \cdot \vec{v_2} \vec{S_1} \cdot \vec{v_1} \vec{S_1} \cdot \vec{v_1} - 10 \hat{n} \cdot \vec{v_1} \vec{S_1} \cdot \vec{v_2} \vec{S_1} \cdot \vec{v_1} + \right. \right. \\ \left. \left. 2 \hat{n} \cdot \vec{v_2} \vec{S_1} \cdot \vec{v_2} \vec{S_1} \cdot \vec{v_1} + 6 \hat{n} \cdot \vec{v_2} \vec{S_1} \cdot \vec{a_1} \vec{S_1} \cdot \vec{v_1} - \hat{n} \cdot \vec{v_1} \vec{S_1} \cdot \vec{a_2} \vec{S_1} \cdot \vec{v_1} - 12 \hat{n} \cdot \vec{v_1} \vec{S_1} \cdot \vec{a_1} \vec{S_1} \cdot \vec{v_2} - \right. \right. \\ \left. \left. 4 \hat{n} \cdot \vec{a_1} \vec{S_1} \cdot \vec{v_1} \vec{S_1} \cdot \vec{v_2} - 6 \hat{n} \cdot \vec{v_2} \vec{S_1} \cdot \vec{S_1} \vec{v_1} \cdot \vec{a_1} + 2 \hat{n} \cdot \vec{v_1} \vec{S_1} \cdot \vec{S_1} \vec{v_1} \cdot \vec{a_2} - 6 \hat{n} \cdot \vec{v_2} \vec{S_1} \cdot \vec{S_1} \vec{v_1} \cdot \vec{v_1} + \right. \right. \\ \left. \left. \frac{13}{2} \hat{n} \cdot \vec{v_1} \vec{S_1} \cdot \vec{S_1} \vec{v_1} \cdot \vec{v_2} - 4 \hat{n} \cdot \vec{v_2} \vec{S_1} \cdot \vec{S_1} \vec{v_1} \cdot \vec{v_2} + \frac{7}{2} \hat{n} \cdot \vec{S_1} \vec{S_1} \cdot \vec{v_1} \vec{v_1} \cdot \vec{v_2} + \hat{n} \cdot \vec{S_1} \vec{S_1} \cdot \vec{v_2} \vec{v_1} \cdot \vec{v_2} \right) + \right. \\ \left. \frac{1}{r^4} \left( 10 \vec{v_1} \cdot \vec{v_2} \left( \hat{n} \times \vec{S_1} \cdot \vec{v_1} \right)^2 + 24 \hat{n} \times \vec{S_1} \cdot \vec{v_2} \left( \hat{n} \cdot \vec{v_1} \right)^2 \hat{n} \times \vec{S_1} \cdot \vec{v_1} + 8 \vec{S_1} \times \vec{v_1} \cdot \vec{v_2} \hat{n} \cdot \vec{v_1} \hat{n} \times \vec{S_1} \cdot \vec{v_1} - \right. \right. \\ \left. \left. 4 \vec{S_1} \times \vec{v_1} \cdot \vec{v_2} \hat{n} \cdot \vec{v_2} \hat{n} \times \vec{S_1} \cdot \vec{v_1} - 12 \hat{n} \times \vec{S_1} \cdot \vec{v_2} \hat{n} \cdot \vec{v_1} \hat{n} \cdot \vec{v_2} \hat{n} \times \vec{S_1} \cdot \vec{v_1} - 12 \hat{n} \times \vec{S_1} \cdot \vec{v_2} \vec{v_1} \cdot \vec{v_1} \hat{n} \times \vec{S_1} \cdot \vec{v_1} + \right. \right. \\ \left. \left. 2 \hat{n} \times \vec{S_1} \cdot \vec{v_2} \vec{v_1} \cdot \vec{v_2} \hat{n} \times \vec{S_1} \cdot \vec{v_1} + \left( \vec{S_1} \times \vec{v_1} \cdot \vec{v_2} \right)^2 - 3 \hat{n} \cdot \vec{v_1} \hat{n} \cdot \vec{v_2} \left( \vec{S_1} \cdot \vec{v_1} \right)^2 - 2 \left( \hat{n} \cdot \vec{S_1} \right)^2 \left( \vec{v_1} \cdot \vec{v_2} \right)^2 - \right. \right. \\ \left. \left. 2 \vec{S_1} \cdot \vec{S_1} \left( \vec{v_1} \cdot \vec{v_2} \right)^2 + 2 \hat{n} \times \vec{S_1} \cdot \vec{v_2} \vec{S_1} \times \vec{v_1} \cdot \vec{v_2} \hat{n} \cdot \vec{v_1} + 6 \left( \hat{n} \cdot \vec{v_1} \right)^2 \vec{S_1} \cdot \vec{v_1} \vec{S_1} \cdot \vec{v_2} - 4 \hat{n} \cdot \vec{v_1} \hat{n} \cdot \vec{v_2} \vec{S_1} \cdot \vec{v_1} \vec{S_1} \cdot \vec{v_2} - \right. \right. \\ \left. \left. 2 \hat{n} \cdot \vec{v_1} \hat{n} \cdot \vec{v_2} \vec{S_1} \cdot \vec{S_1} \vec{v_1} \cdot \vec{v_1} + 5 \hat{n} \cdot \vec{S_1} \hat{n} \cdot \vec{v_2} \vec{S_1} \cdot \vec{v_1} \vec{v_1} \cdot \vec{v_1} - \frac{9}{2} \vec{S_1} \cdot \vec{v_1} \vec{S_1} \cdot \vec{v_2} \vec{v_1} \cdot \vec{v_1} + \frac{3}{2} \left( \vec{S_1} \cdot \vec{v_1} \right)^2 \vec{v_1} \cdot \vec{v_2} + \right. \right. \\ \left. \left. 12 \left( \hat{n} \cdot \vec{S_1} \right)^2 \hat{n} \cdot \vec{v_1} \hat{n} \cdot \vec{v_2} \vec{v_1} \cdot \vec{v_2} - 10 \left( \hat{n} \cdot \vec{v_1} \right)^2 \vec{S_1} \cdot \vec{S_1} \vec{v_1} \cdot \vec{v_2} + 8 \hat{n} \cdot \vec{v_1} \hat{n} \cdot \vec{v_2} \vec{S_1} \cdot \vec{S_1} \vec{v_1} \cdot \vec{v_2} + \right. \right. \\ \left. \left. 4 \hat{n} \cdot \vec{S_1} \hat{n} \cdot \vec{v_1} \vec{S_1} \cdot \vec{v_1} \vec{v_1} \cdot \vec{v_2} - 4 \hat{n} \cdot \vec{S_1} \hat{n} \cdot \vec{v_2} \vec{S_1} \cdot \vec{v_1} \vec{v_1} \cdot \vec{v_2} - 4 \hat{n} \cdot \vec{S_1} \hat{n} \cdot \vec{v_1} \vec{S_1} \cdot \vec{v_2} \vec{v_1} \cdot \vec{v_2} + \right. \right. \\ \left. \left. 2 \vec{S_1} \cdot \vec{v_1} \vec{S_1} \cdot \vec{v_2} \vec{v_1} \cdot \vec{v_2} + 3 \vec{S_1} \cdot \vec{S_1} \vec{v_1} \cdot \vec{v_1} \vec{v_1} \cdot \vec{v_2} - 5 \hat{n} \cdot \vec{v_1} \hat{n} \cdot \vec{v_2} \vec{S_1} \cdot \vec{S_1} \vec{v_2} \cdot \vec{v_2} + 3 \hat{n} \cdot \vec{S_1} \hat{n} \cdot \vec{v_2} \vec{S_1} \cdot \vec{v_1} \vec{v_2} \cdot \vec{v_2} + \right. \right. \\ \left. \left. 2 \hat{n} \cdot \vec{S_1} \hat{n} \cdot \vec{v_1} \vec{S_1} \cdot \vec{v_2} \vec{v_2} \cdot \vec{v_2} - \frac{3}{2} \vec{S_1} \cdot \vec{v_1} \vec{S_1} \cdot \vec{v_2} \vec{v_2} \cdot \vec{v_2} - \left( \hat{n} \cdot \vec{S_1} \right)^2 \vec{v_1} \cdot \vec{v_2} \vec{v_2} \cdot \vec{v_2} + \frac{3}{2} \vec{S_1} \cdot \vec{S_1} \vec{v_1} \cdot \vec{v_2} \vec{v_2} \cdot \vec{v_2} \right) \right\} m_2 \Bigg\}$$

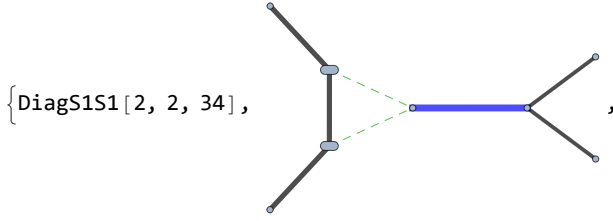

$$G^2 \left( \frac{\frac{1}{2} \left( \hat{n} \times \vec{S}_1 \cdot \vec{v}_2 \right)^2 + \frac{1}{2} \left( \vec{S}_1 \cdot \vec{v}_2 \right)^2 - \frac{1}{2} \vec{S}_1 \cdot \vec{S}_1 \vec{v}_2 \cdot \vec{v}_2}{r^2} + \frac{1}{r^3} \left( -4 \hat{n} \cdot \vec{v}_1 \vec{S}_1 \cdot \vec{S}_1 (\hat{n} \cdot \vec{v}_2)^2 + \right. \right.$$

$$4 \hat{n} \cdot \vec{S}_1 \vec{S}_1 \cdot \vec{a}_1 (\hat{n} \cdot \vec{v}_2)^2 - 4 \hat{n} \cdot \vec{a}_1 \vec{S}_1 \cdot \vec{S}_1 (\hat{n} \cdot \vec{v}_2)^2 + 4 \hat{n} \cdot \vec{S}_1 \vec{S}_1 \cdot \vec{v}_1 (\hat{n} \cdot \vec{v}_2)^2 - 3 \hat{n} \times \vec{S}_1 \cdot \vec{v}_2 \vec{S}_1 \times \vec{v}_1 \cdot \vec{v}_2 -$$

$$2 \hat{n} \times \vec{S}_1 \cdot \vec{v}_2 \vec{S}_1 \times \vec{a}_1 \cdot \vec{v}_2 - 2 \hat{n} \times \vec{S}_1 \cdot \vec{v}_2 \hat{n} \times \vec{S}_1 \cdot \vec{v}_2 \hat{n} \cdot \vec{v}_1 - \hat{n} \cdot \vec{v}_1 \vec{S}_1 \cdot \vec{v}_2 \vec{S}_1 \cdot \vec{v}_2 + \hat{n} \cdot \vec{v}_1 \vec{S}_1 \cdot \vec{S}_1 \vec{v}_2 \cdot \vec{v}_2 \left. \right) + \frac{1}{r^4}$$

$$\left( -\frac{27}{4} (\hat{n} \cdot \vec{v}_2)^2 (\hat{n} \times \vec{S}_1 \cdot \vec{v}_1)^2 + \frac{5}{4} \vec{v}_2 \cdot \vec{v}_2 (\hat{n} \times \vec{S}_1 \cdot \vec{v}_1)^2 + \vec{S}_1 \times \vec{v}_1 \cdot \vec{v}_2 \hat{n} \cdot \vec{v}_2 \hat{n} \times \vec{S}_1 \cdot \vec{v}_1 + \hat{n} \times \vec{S}_1 \cdot \vec{v}_2 \vec{v}_1 \cdot \vec{v}_2 \hat{n} \times \vec{S}_1 \cdot \vec{v}_1 + \right.$$

$$(\vec{S}_1 \times \vec{v}_1 \cdot \vec{v}_2)^2 + \frac{9}{4} (\hat{n} \times \vec{S}_1 \cdot \vec{v}_2)^2 (\hat{n} \cdot \vec{v}_1)^2 - \frac{3}{2} (\hat{n} \cdot \vec{v}_2)^2 (\vec{S}_1 \cdot \vec{v}_1)^2 + \frac{3}{4} (\hat{n} \cdot \vec{v}_1)^2 (\vec{S}_1 \cdot \vec{v}_2)^2 +$$

$$\vec{S}_1 \cdot \vec{S}_1 (\vec{v}_1 \cdot \vec{v}_2)^2 - \frac{7}{8} (\hat{n} \cdot \vec{S}_1)^2 (\vec{v}_2 \cdot \vec{v}_2)^2 + \frac{5}{8} \vec{S}_1 \cdot \vec{S}_1 (\vec{v}_2 \cdot \vec{v}_2)^2 + 4 \hat{n} \times \vec{S}_1 \cdot \vec{v}_2 \vec{S}_1 \times \vec{v}_1 \cdot \vec{v}_2 \hat{n} \cdot \vec{v}_1 +$$

$$\frac{9}{4} (\hat{n} \cdot \vec{v}_1)^2 (\hat{n} \cdot \vec{v}_2)^2 \vec{S}_1 \cdot \vec{S}_1 - \frac{9}{4} \hat{n} \cdot \vec{S}_1 \hat{n} \cdot \vec{v}_1 (\hat{n} \cdot \vec{v}_2)^2 \vec{S}_1 \cdot \vec{v}_1 - \frac{1}{2} \hat{n} \cdot \vec{v}_1 \hat{n} \cdot \vec{v}_2 \vec{S}_1 \cdot \vec{v}_1 \vec{S}_1 \cdot \vec{v}_2 -$$

$$\frac{3}{4} (\hat{n} \times \vec{S}_1 \cdot \vec{v}_2)^2 \vec{v}_1 \cdot \vec{v}_1 - \frac{1}{4} (\vec{S}_1 \cdot \vec{v}_2)^2 \vec{v}_1 \cdot \vec{v}_1 + \frac{3}{2} (\hat{n} \cdot \vec{v}_2)^2 \vec{S}_1 \cdot \vec{S}_1 \vec{v}_1 \cdot \vec{v}_1 - 3 \hat{n} \cdot \vec{v}_1 \hat{n} \cdot \vec{v}_2 \vec{S}_1 \cdot \vec{S}_1 \vec{v}_1 \cdot \vec{v}_2 +$$

$$\frac{7}{2} \hat{n} \cdot \vec{S}_1 \hat{n} \cdot \vec{v}_2 \vec{S}_1 \cdot \vec{v}_1 \vec{v}_1 \cdot \vec{v}_2 - \vec{S}_1 \cdot \vec{v}_1 \vec{S}_1 \cdot \vec{v}_2 \vec{v}_1 \cdot \vec{v}_2 - \frac{1}{2} (\hat{n} \times \vec{S}_1 \cdot \vec{v}_2)^2 \vec{v}_2 \cdot \vec{v}_2 + \frac{9}{8} (\hat{n} \cdot \vec{S}_1)^2 (\hat{n} \cdot \vec{v}_2)^2 \vec{v}_2 \cdot \vec{v}_2 +$$

$$\frac{3}{2} (\vec{S}_1 \cdot \vec{v}_1)^2 \vec{v}_2 \cdot \vec{v}_2 - \frac{1}{2} (\vec{S}_1 \cdot \vec{v}_2)^2 \vec{v}_2 \cdot \vec{v}_2 + \frac{3}{2} (\hat{n} \cdot \vec{v}_1)^2 \vec{S}_1 \cdot \vec{S}_1 \vec{v}_2 \cdot \vec{v}_2 - \frac{7}{8} (\hat{n} \cdot \vec{v}_2)^2 \vec{S}_1 \cdot \vec{S}_1 \vec{v}_2 \cdot \vec{v}_2 -$$

$$\left. \frac{9}{4} \hat{n} \cdot \vec{S}_1 \hat{n} \cdot \vec{v}_1 \vec{S}_1 \cdot \vec{v}_1 \vec{v}_2 \cdot \vec{v}_2 + \frac{1}{2} \hat{n} \cdot \vec{S}_1 \hat{n} \cdot \vec{v}_2 \vec{S}_1 \cdot \vec{v}_2 \vec{v}_2 \cdot \vec{v}_2 - \frac{5}{4} \vec{S}_1 \cdot \vec{S}_1 \vec{v}_1 \cdot \vec{v}_1 \vec{v}_2 \cdot \vec{v}_2 \right) m_2 \Bigg\}$$

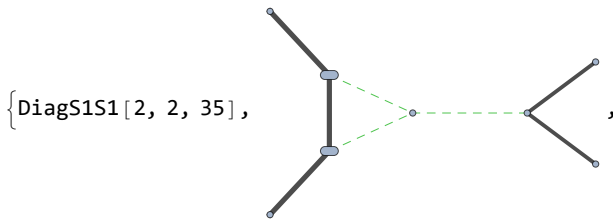

$$G^2 \left( \frac{1}{r^2} \left( -8 \hat{n} \times \vec{S}_1 \cdot \vec{v}_1 \hat{n} \times \vec{S}_1 \cdot \vec{v}_2 - 8 \hat{n} \times \vec{S}_1 \cdot \vec{a}_1 \hat{n} \times \vec{S}_1 \cdot \vec{v}_2 + 6 \hat{n} \times \vec{S}_1 \cdot \vec{v}_1 \hat{n} \times \vec{S}_1 \cdot \vec{a}_2 + 6 \hat{n} \times \vec{S}_1 \cdot \vec{a}_1 \hat{n} \times \vec{S}_1 \cdot \vec{a}_2 - \right. \right.$$

$$2 \hat{n} \cdot \vec{v}_1 \hat{n} \cdot \vec{v}_2 \vec{S}_1 \cdot \vec{S}_1 + 2 \hat{n} \cdot \vec{S}_1 \hat{n} \cdot \vec{v}_2 \vec{S}_1 \cdot \vec{a}_1 + 2 \hat{n} \cdot \vec{S}_1 \hat{n} \cdot \vec{v}_2 \vec{S}_1 \cdot \vec{v}_1 - 6 \vec{S}_1 \cdot \vec{v}_1 \vec{S}_1 \cdot \vec{v}_2 + 6 \hat{n} \cdot \vec{S}_1 \hat{n} \cdot \vec{v}_2 \vec{S}_1 \cdot \vec{a}_1 -$$

$$14 \hat{n} \cdot \vec{a}_1 \hat{n} \cdot \vec{v}_2 \vec{S}_1 \cdot \vec{S}_1 + 10 \vec{a}_1 \cdot \vec{v}_2 \vec{S}_1 \cdot \vec{S}_1 - 6 \hat{n} \cdot \vec{v}_1 \hat{n} \cdot \vec{v}_2 \vec{S}_1 \cdot \vec{S}_1 + 12 \hat{n} \cdot \vec{S}_1 \hat{n} \cdot \vec{v}_2 \vec{S}_1 \cdot \vec{a}_1 - 4 \vec{S}_1 \cdot \vec{v}_2 \vec{S}_1 \cdot \vec{a}_1 +$$

$$2 \vec{S}_1 \cdot \vec{a}_1 \vec{S}_1 \cdot \vec{a}_2 - 6 \hat{n} \cdot \vec{a}_1 \hat{n} \cdot \vec{v}_2 \vec{S}_1 \cdot \vec{S}_1 + 2 \vec{a}_1 \cdot \vec{v}_2 \vec{S}_1 \cdot \vec{S}_1 - 2 \vec{a}_1 \cdot \vec{a}_2 \vec{S}_1 \cdot \vec{S}_1 + 6 \hat{n} \cdot \vec{S}_1 \hat{n} \cdot \vec{v}_2 \vec{S}_1 \cdot \vec{v}_1 + 2 \vec{S}_1 \cdot \vec{a}_2 \vec{S}_1 \cdot \vec{v}_1 -$$

$$2 \vec{S}_1 \cdot \vec{v}_2 \vec{S}_1 \cdot \vec{v}_1 - 6 \vec{S}_1 \cdot \vec{a}_1 \vec{S}_1 \cdot \vec{v}_2 - 2 \vec{S}_1 \cdot \vec{a}_1 \vec{S}_1 \cdot \vec{v}_2 - 2 \vec{S}_1 \cdot \vec{S}_1 \vec{v}_1 \cdot \vec{a}_2 + 6 \vec{S}_1 \cdot \vec{S}_1 \vec{v}_1 \cdot \vec{v}_2 + 2 \vec{S}_1 \cdot \vec{S}_1 \vec{v}_1 \cdot \vec{v}_2 \left. \right) +$$

$$\frac{1}{r^3} \left( 10 \hat{n} \cdot \vec{v}_2 \vec{S}_1 \cdot \vec{S}_1 (\hat{n} \cdot \vec{v}_1)^2 + 8 \hat{n} \times \vec{S}_1 \cdot \vec{v}_2 \hat{n} \times \vec{S}_1 \cdot \vec{v}_1 \hat{n} \cdot \vec{v}_1 - 4 \hat{n} \times \vec{S}_1 \cdot \vec{a}_2 \hat{n} \times \vec{S}_1 \cdot \vec{v}_1 \hat{n} \cdot \vec{v}_1 + \right.$$

[illegible]

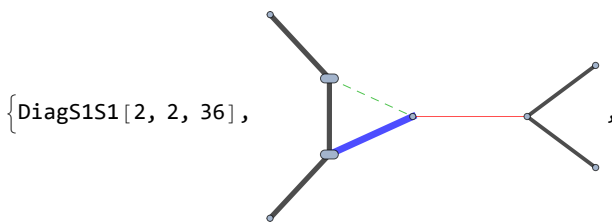

$$G^2 \left( \frac{1}{r^2} \left( 6 \left( \hat{n} \times \vec{S_1} \cdot \vec{v_1} \right)^2 + 8 \hat{n} \times \vec{S_1} \cdot \vec{a_1} \hat{n} \times \vec{S_1} \cdot \vec{v_1} + 4 \hat{n} \times \vec{S_1} \cdot \vec{a_1} \hat{n} \times \vec{S_1} \cdot \vec{v_1} - 6 \left( \hat{n} \cdot \vec{v_1} \right)^2 \vec{S_1} \cdot \vec{S_1} + 8 \hat{n} \cdot \vec{S_1} \hat{n} \cdot \vec{v_1} \vec{S_1} \cdot \vec{a_1} + \right. \right. \\ \left. \left. 4 \hat{n} \cdot \vec{a_1} \hat{n} \cdot \vec{S_1} \vec{S_1} \cdot \vec{v_1} + 6 \hat{n} \cdot \vec{S_1} \hat{n} \cdot \vec{v_1} \vec{S_1} \cdot \vec{v_1} + 8 \hat{n} \cdot \vec{S_1} \hat{n} \cdot \vec{v_1} \vec{S_1} \cdot \vec{a_1} - 28 \hat{n} \cdot \vec{a_1} \hat{n} \cdot \vec{v_1} \vec{S_1} \cdot \vec{S_1} - \right. \right. \\ \left. \left. 8 \left( \hat{n} \cdot \vec{v_1} \right)^2 \vec{S_1} \cdot \vec{S_1} + 16 \hat{n} \cdot \vec{S_1} \hat{n} \cdot \vec{v_1} \vec{S_1} \cdot \vec{a_1} - 8 \vec{S_1} \cdot \vec{v_1} \vec{S_1} \cdot \vec{a_1} - 8 \hat{n} \cdot \vec{a_1} \hat{n} \cdot \vec{v_1} \vec{S_1} \cdot \vec{S_1} + 8 \hat{n} \cdot \vec{S_1} \hat{n} \cdot \vec{v_1} \vec{S_1} \cdot \vec{v_1} - \right. \right. \\ \left. \left. 4 \vec{S_1} \cdot \vec{v_1} \vec{S_1} \cdot \vec{v_1} - 4 \vec{S_1} \cdot \vec{a_1} \vec{S_1} \cdot \vec{v_1} + 4 \vec{S_1} \cdot \vec{S_1} \vec{v_1} \cdot \vec{a_1} + 8 \vec{S_1} \cdot \vec{S_1} \vec{v_1} \cdot \vec{a_1} + 4 \vec{S_1} \cdot \vec{S_1} \vec{v_1} \cdot \vec{v_1} \right) + \frac{1}{r^3} \right.$$

$$\begin{aligned}
& \left( 30 \vec{S}_1 \cdot \vec{S}_1 (\hat{n} \cdot \vec{v}_1)^3 - 2 \hat{n} \cdot \vec{S}_1 \vec{S}_1 \cdot \vec{v}_1 (\hat{n} \cdot \vec{v}_1)^2 - 26 \hat{n} \cdot \vec{v}_2 \vec{S}_1 \cdot \vec{S}_1 (\hat{n} \cdot \vec{v}_1)^2 - 34 \hat{n} \cdot \vec{S}_1 \vec{S}_1 \cdot \vec{a}_1 (\hat{n} \cdot \vec{v}_1)^2 + \right. \\
& 48 \hat{n} \cdot \vec{a}_1 \vec{S}_1 \cdot \vec{S}_1 (\hat{n} \cdot \vec{v}_1)^2 - 28 \hat{n} \cdot \vec{S}_1 \vec{S}_1 \cdot \vec{v}_1 (\hat{n} \cdot \vec{v}_1)^2 - 30 \hat{n} \times \vec{S}_1 \cdot \vec{v}_1 \hat{n} \times \vec{S}_1 \cdot \vec{v}_1 \hat{n} \cdot \vec{v}_1 - \\
& 48 \hat{n} \times \vec{S}_1 \cdot \vec{a}_1 \hat{n} \times \vec{S}_1 \cdot \vec{v}_1 \hat{n} \cdot \vec{v}_1 + 32 \hat{n} \cdot \vec{S}_1 \hat{n} \cdot \vec{v}_2 \vec{S}_1 \cdot \vec{a}_1 \hat{n} \cdot \vec{v}_1 - 44 \hat{n} \cdot \vec{a}_1 \hat{n} \cdot \vec{v}_2 \vec{S}_1 \cdot \vec{S}_1 \hat{n} \cdot \vec{v}_1 + \\
& 11 \vec{a}_1 \cdot \vec{v}_2 \vec{S}_1 \cdot \vec{S}_1 \hat{n} \cdot \vec{v}_1 - 14 \hat{n} \cdot \vec{a}_1 \hat{n} \cdot \vec{S}_1 \vec{S}_1 \cdot \vec{v}_1 \hat{n} \cdot \vec{v}_1 + 26 \hat{n} \cdot \vec{S}_1 \hat{n} \cdot \vec{v}_2 \vec{S}_1 \cdot \vec{v}_1 \hat{n} \cdot \vec{v}_1 + \frac{13}{2} \vec{S}_1 \cdot \vec{v}_1 \vec{S}_1 \cdot \vec{v}_1 \hat{n} \cdot \vec{v}_1 - \\
& \frac{13}{2} \vec{S}_1 \cdot \vec{v}_2 \vec{S}_1 \cdot \vec{v}_1 \hat{n} \cdot \vec{v}_1 + \frac{13}{2} \vec{S}_1 \cdot \vec{a}_1 \vec{S}_1 \cdot \vec{v}_1 \hat{n} \cdot \vec{v}_1 - 8 \vec{S}_1 \cdot \vec{a}_1 \vec{S}_1 \cdot \vec{v}_2 \hat{n} \cdot \vec{v}_1 - \frac{17}{2} \vec{S}_1 \cdot \vec{S}_1 \vec{v}_1 \cdot \vec{a}_1 \hat{n} \cdot \vec{v}_1 - \\
& \frac{25}{2} \vec{S}_1 \cdot \vec{S}_1 \vec{v}_1 \cdot \vec{v}_1 \hat{n} \cdot \vec{v}_1 + 13 \vec{S}_1 \cdot \vec{S}_1 \vec{v}_1 \cdot \vec{v}_2 \hat{n} \cdot \vec{v}_1 + 6 (\hat{n} \cdot \vec{S}_1)^2 \vec{v}_2 \cdot \vec{a}_2 \hat{n} \cdot \vec{v}_1 + 6 \vec{S}_1 \cdot \vec{S}_1 \vec{v}_2 \cdot \vec{a}_2 \hat{n} \cdot \vec{v}_1 + \\
& 6 \hat{n} \cdot \vec{S}_1 \hat{n} \cdot \vec{S}_1 \vec{v}_2 \cdot \vec{v}_2 \hat{n} \cdot \vec{v}_1 + \frac{9}{2} \vec{S}_1 \cdot \vec{S}_1 \vec{v}_2 \cdot \vec{v}_2 \hat{n} \cdot \vec{v}_1 + \frac{5}{2} \hat{n} \cdot \vec{a}_1 (\vec{S}_1 \cdot \vec{v}_1)^2 - \frac{9}{2} \hat{n} \times \vec{S}_1 \cdot \vec{v}_1 \vec{S}_1 \times \vec{v}_1 \cdot \vec{v}_2 - \\
& 9 \hat{n} \times \vec{S}_1 \cdot \vec{v}_1 \vec{S}_1 \times \vec{a}_1 \cdot \vec{v}_2 - \frac{17}{2} \hat{n} \times \vec{S}_1 \cdot \vec{v}_1 \vec{S}_1 \times \vec{v}_1 \cdot \vec{a}_1 - \frac{9}{2} \hat{n} \times \vec{S}_1 \cdot \vec{v}_1 \vec{S}_1 \times \vec{v}_1 \cdot \vec{v}_2 - 9 \hat{n} \times \vec{S}_1 \cdot \vec{a}_1 \vec{S}_1 \times \vec{v}_1 \cdot \vec{v}_2 + \\
& 18 \hat{n} \times \vec{S}_1 \cdot \vec{v}_1 \hat{n} \times \vec{S}_1 \cdot \vec{v}_1 \hat{n} \cdot \vec{v}_2 + 36 \hat{n} \times \vec{S}_1 \cdot \vec{a}_1 \hat{n} \times \vec{S}_1 \cdot \vec{v}_1 \hat{n} \cdot \vec{v}_2 + 12 \hat{n} \cdot \vec{a}_1 \hat{n} \cdot \vec{S}_1 \hat{n} \cdot \vec{v}_2 \vec{S}_1 \cdot \vec{v}_1 - 4 \hat{n} \cdot \vec{v}_2 \vec{S}_1 \cdot \vec{v}_1 \vec{S}_1 \cdot \vec{v}_1 - \\
& 3 \hat{n} \cdot \vec{S}_1 \vec{a}_1 \cdot \vec{v}_2 \vec{S}_1 \cdot \vec{v}_1 - 4 \hat{n} \cdot \vec{v}_2 \vec{S}_1 \cdot \vec{a}_1 \vec{S}_1 \cdot \vec{v}_1 - 3 \hat{n} \cdot \vec{a}_1 \vec{S}_1 \cdot \vec{v}_1 \vec{S}_1 \cdot \vec{v}_2 + 4 \hat{n} \cdot \vec{v}_2 \vec{S}_1 \cdot \vec{S}_1 \vec{v}_1 \cdot \vec{a}_1 + \\
& 2 \hat{n} \cdot \vec{S}_1 \vec{S}_1 \cdot \vec{v}_1 \vec{v}_1 \cdot \vec{a}_1 + \frac{1}{2} \hat{n} \cdot \vec{S}_1 \vec{S}_1 \cdot \vec{v}_1 \vec{v}_1 \cdot \vec{v}_1 + 4 \hat{n} \cdot \vec{v}_2 \vec{S}_1 \cdot \vec{S}_1 \vec{v}_1 \cdot \vec{v}_1 + 7 \hat{n} \cdot \vec{S}_1 \vec{S}_1 \cdot \vec{a}_1 \vec{v}_1 \cdot \vec{v}_1 - \\
& \frac{19}{2} \hat{n} \cdot \vec{a}_1 \vec{S}_1 \cdot \vec{S}_1 \vec{v}_1 \cdot \vec{v}_1 + \frac{11}{2} \hat{n} \cdot \vec{S}_1 \vec{S}_1 \cdot \vec{v}_1 \vec{v}_1 \cdot \vec{v}_1 - 8 \hat{n} \cdot \vec{S}_1 \vec{S}_1 \cdot \vec{a}_1 \vec{v}_1 \cdot \vec{v}_2 + 11 \hat{n} \cdot \vec{a}_1 \vec{S}_1 \cdot \vec{S}_1 \vec{v}_1 \cdot \vec{v}_2 - \\
& \frac{13}{2} \hat{n} \cdot \vec{S}_1 \vec{S}_1 \cdot \vec{v}_1 \vec{v}_1 \cdot \vec{v}_2 - 6 \hat{n} \cdot \vec{S}_1 \vec{S}_1 \cdot \vec{v}_1 \vec{v}_2 \cdot \vec{a}_2 - \frac{3}{2} \hat{n} \cdot \vec{S}_1 \vec{S}_1 \cdot \vec{v}_1 \vec{v}_2 \cdot \vec{v}_2 - 3 \hat{n} \cdot \vec{S}_1 \vec{S}_1 \cdot \vec{v}_1 \vec{v}_2 \cdot \vec{v}_2 \Big) + \frac{1}{r^4} \\
& \left( -12 \vec{S}_1 \cdot \vec{S}_1 (\hat{n} \cdot \vec{v}_1)^4 + 12 \hat{n} \cdot \vec{v}_2 \vec{S}_1 \cdot \vec{S}_1 (\hat{n} \cdot \vec{v}_1)^3 + 12 \hat{n} \cdot \vec{S}_1 \vec{S}_1 \cdot \vec{v}_1 (\hat{n} \cdot \vec{v}_1)^3 + 36 (\hat{n} \times \vec{S}_1 \cdot \vec{v}_1)^2 (\hat{n} \cdot \vec{v}_1)^2 + \right. \\
& 3 (\vec{S}_1 \cdot \vec{v}_1)^2 (\hat{n} \cdot \vec{v}_1)^2 - 12 \hat{n} \cdot \vec{S}_1 \hat{n} \cdot \vec{v}_2 \vec{S}_1 \cdot \vec{v}_1 (\hat{n} \cdot \vec{v}_1)^2 + 2 \vec{S}_1 \cdot \vec{v}_1 \vec{S}_1 \cdot \vec{v}_2 (\hat{n} \cdot \vec{v}_1)^2 - \\
& 6 \vec{S}_1 \cdot \vec{S}_1 \vec{v}_1 \cdot \vec{v}_2 (\hat{n} \cdot \vec{v}_1)^2 - 18 (\hat{n} \cdot \vec{S}_1)^2 \vec{v}_2 \cdot \vec{v}_2 (\hat{n} \cdot \vec{v}_1)^2 - 9 \vec{S}_1 \cdot \vec{S}_1 \vec{v}_2 \cdot \vec{v}_2 (\hat{n} \cdot \vec{v}_1)^2 - 4 \hat{n} \cdot \vec{v}_2 (\vec{S}_1 \cdot \vec{v}_1)^2 \hat{n} \cdot \vec{v}_1 + \\
& 12 \hat{n} \times \vec{S}_1 \cdot \vec{v}_1 \vec{S}_1 \times \vec{v}_1 \cdot \vec{v}_2 \hat{n} \cdot \vec{v}_1 - 36 (\hat{n} \times \vec{S}_1 \cdot \vec{v}_1)^2 \hat{n} \cdot \vec{v}_2 \hat{n} \cdot \vec{v}_1 + 8 \hat{n} \cdot \vec{v}_2 \vec{S}_1 \cdot \vec{S}_1 \vec{v}_1 \cdot \vec{v}_1 \hat{n} \cdot \vec{v}_1 - \\
& 3 \hat{n} \cdot \vec{S}_1 \vec{S}_1 \cdot \vec{v}_1 \vec{v}_1 \cdot \vec{v}_1 \hat{n} \cdot \vec{v}_1 + 4 \hat{n} \cdot \vec{S}_1 \vec{S}_1 \cdot \vec{v}_1 \vec{v}_1 \cdot \vec{v}_2 \hat{n} \cdot \vec{v}_1 + 18 (\hat{n} \cdot \vec{S}_1)^2 \hat{n} \cdot \vec{v}_2 \vec{v}_2 \cdot \vec{v}_2 \hat{n} \cdot \vec{v}_1 + \\
& 12 \hat{n} \cdot \vec{v}_2 \vec{S}_1 \cdot \vec{S}_1 \vec{v}_2 \cdot \vec{v}_2 \hat{n} \cdot \vec{v}_1 + 15 \hat{n} \cdot \vec{S}_1 \vec{S}_1 \cdot \vec{v}_1 \vec{v}_2 \cdot \vec{v}_2 \hat{n} \cdot \vec{v}_1 - 6 \hat{n} \cdot \vec{S}_1 \vec{S}_1 \cdot \vec{v}_2 \vec{v}_2 \cdot \vec{v}_2 \hat{n} \cdot \vec{v}_1 + \\
& \vec{S}_1 \cdot \vec{S}_1 (\vec{v}_1 \cdot \vec{v}_1)^2 - 4 (\hat{n} \times \vec{S}_1 \cdot \vec{v}_1)^2 \vec{v}_1 \cdot \vec{v}_1 - (\vec{S}_1 \cdot \vec{v}_1)^2 \vec{v}_1 \cdot \vec{v}_1 - 4 \hat{n} \cdot \vec{S}_1 \hat{n} \cdot \vec{v}_2 \vec{S}_1 \cdot \vec{v}_1 \vec{v}_1 \cdot \vec{v}_1 + \\
& \vec{S}_1 \cdot \vec{v}_1 \vec{S}_1 \cdot \vec{v}_2 \vec{v}_1 \cdot \vec{v}_1 + 6 (\hat{n} \times \vec{S}_1 \cdot \vec{v}_1)^2 \vec{v}_1 \cdot \vec{v}_2 + (\vec{S}_1 \cdot \vec{v}_1)^2 \vec{v}_1 \cdot \vec{v}_2 - 2 \vec{S}_1 \cdot \vec{S}_1 \vec{v}_1 \cdot \vec{v}_1 \vec{v}_1 \cdot \vec{v}_2 + \\
& 3 (\hat{n} \times \vec{S}_1 \cdot \vec{v}_1)^2 \vec{v}_2 \cdot \vec{v}_2 - \frac{3}{2} (\vec{S}_1 \cdot \vec{v}_1)^2 \vec{v}_2 \cdot \vec{v}_2 - 12 \hat{n} \cdot \vec{S}_1 \hat{n} \cdot \vec{v}_2 \vec{S}_1 \cdot \vec{v}_1 \vec{v}_2 \cdot \vec{v}_2 + 3 \vec{S}_1 \cdot \vec{v}_1 \vec{S}_1 \cdot \vec{v}_2 \vec{v}_2 \cdot \vec{v}_2 + \\
& 3 (\hat{n} \cdot \vec{S}_1)^2 \vec{v}_1 \cdot \vec{v}_1 \vec{v}_2 \cdot \vec{v}_2 + \frac{3}{2} \vec{S}_1 \cdot \vec{S}_1 \vec{v}_1 \cdot \vec{v}_1 \vec{v}_2 \cdot \vec{v}_2 - 3 (\hat{n} \cdot \vec{S}_1)^2 \vec{v}_1 \cdot \vec{v}_2 \vec{v}_2 \cdot \vec{v}_2 - 3 \vec{S}_1 \cdot \vec{S}_1 \vec{v}_1 \cdot \vec{v}_2 \vec{v}_2 \cdot \vec{v}_2 \Big) \Big\} m_2 \}
\end{aligned}$$

{DiagS1S1[2, 2, 37],

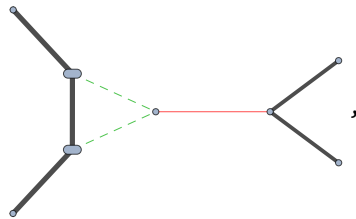

$$\begin{aligned}
& G^2 m_2 \left( \frac{1}{r^3} \left( 9 \vec{S}_1 \times \vec{v}_1 \cdot \vec{a}_1 \hat{n} \times \vec{S}_1 \cdot \vec{v}_1 + 5 \vec{S}_1 \cdot \vec{a}_1 \hat{n} \cdot \vec{v}_1 \vec{S}_1 \cdot \vec{v}_1 - 3 \vec{S}_1 \cdot \vec{S}_1 \vec{v}_1 \cdot \vec{a}_1 \hat{n} \cdot \vec{v}_1 - 2 \vec{v}_1 \cdot \vec{a}_1 \hat{n} \cdot \vec{S}_1 \vec{S}_1 \cdot \vec{v}_1 - \right. \right. \\
& \left. \left. \vec{v}_1 \cdot \vec{v}_1 \vec{S}_1 \cdot \vec{a}_1 \hat{n} \cdot \vec{S}_1 + \vec{S}_1 \cdot \vec{S}_1 \vec{v}_1 \cdot \vec{v}_1 \hat{n} \cdot \vec{a}_1 - 3 \vec{v}_2 \cdot \vec{v}_2 \vec{S}_1 \cdot \vec{a}_1 \hat{n} \cdot \vec{S}_1 + 3 \vec{S}_1 \cdot \vec{S}_1 \vec{v}_2 \cdot \vec{v}_2 \hat{n} \cdot \vec{a}_1 + 5 \hat{n} \cdot \vec{v}_1 \vec{S}_1 \cdot \vec{v}_1 \vec{S}_1 \cdot \vec{v}_1 - \right. \right.
\end{aligned}$$

$$\begin{aligned}
& 4 \vec{S}_1 \cdot \vec{S}_1 \vec{v}_1 \cdot \vec{v}_1 \hat{n} \cdot \vec{v}_1 - \vec{v}_1 \cdot \vec{v}_1 \hat{n} \cdot \vec{S}_1 \vec{S}_1 \cdot \vec{v}_1 + 3 \vec{S}_1 \cdot \vec{S}_1 \vec{v}_2 \cdot \vec{v}_2 \hat{n} \cdot \vec{v}_1 - 3 \vec{v}_2 \cdot \vec{v}_2 \hat{n} \cdot \vec{S}_1 \vec{S}_1 \cdot \vec{v}_1 \Big) + \\
& -8 \vec{S}_1 \cdot \vec{a}_1 \vec{S}_1 \cdot \vec{v}_1 + 8 \vec{S}_1 \cdot \vec{S}_1 \vec{v}_1 \cdot \vec{a}_1 - 4 \left( \vec{S}_1 \cdot \vec{a}_1 \right)^2 + 4 \vec{a}_1 \cdot \vec{a}_1 \vec{S}_1 \cdot \vec{S}_1 - 4 \left( \vec{S}_1 \cdot \vec{v}_1 \right)^2 + 4 \vec{S}_1 \cdot \vec{S}_1 \vec{v}_1 \cdot \vec{v}_1 \\
& \frac{1}{r^2} + \\
& \frac{1}{r^4} \left( 4 \vec{v}_1 \cdot \vec{v}_1 \left( \hat{n} \times \vec{S}_1 \cdot \vec{v}_1 \right)^2 + \frac{3}{2} \vec{v}_2 \cdot \vec{v}_2 \left( \hat{n} \times \vec{S}_1 \cdot \vec{v}_1 \right)^2 - \frac{7}{4} \left( \hat{n} \cdot \vec{v}_1 \right)^2 \left( \vec{S}_1 \cdot \vec{v}_1 \right)^2 + \right. \\
& \frac{7}{8} \left( \vec{v}_2 \cdot \vec{v}_2 \right)^2 \left( \hat{n} \cdot \vec{S}_1 \right)^2 + \frac{7}{4} \vec{v}_1 \cdot \vec{v}_1 \hat{n} \cdot \vec{S}_1 \hat{n} \cdot \vec{v}_1 \vec{S}_1 \cdot \vec{v}_1 - \frac{9}{2} \vec{S}_1 \cdot \vec{S}_1 \vec{v}_2 \cdot \vec{v}_2 \left( \hat{n} \cdot \vec{v}_1 \right)^2 + \\
& \left. \frac{9}{2} \vec{v}_2 \cdot \vec{v}_2 \hat{n} \cdot \vec{S}_1 \hat{n} \cdot \vec{v}_1 \vec{S}_1 \cdot \vec{v}_1 - \frac{3}{2} \vec{v}_2 \cdot \vec{v}_2 \left( \vec{S}_1 \cdot \vec{v}_1 \right)^2 + \frac{3}{2} \vec{S}_1 \cdot \vec{S}_1 \vec{v}_1 \cdot \vec{v}_1 \vec{v}_2 \cdot \vec{v}_2 \right) \Big\}
\end{aligned}$$

{DiagS1S1[2, 2, 38],

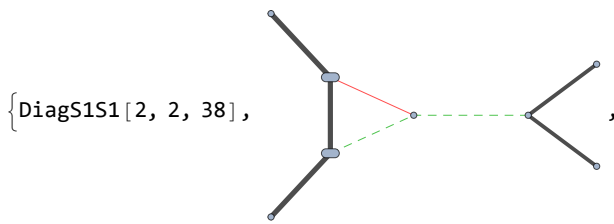

$$\begin{aligned}
& G^2 m_2 \left( \frac{1}{r^3} \left( 16 \vec{S}_1 \times \vec{a}_1 \cdot \vec{v}_2 \hat{n} \times \vec{S}_1 \cdot \vec{v}_1 - 4 \vec{S}_1 \times \vec{v}_1 \cdot \vec{a}_1 \hat{n} \times \vec{S}_1 \cdot \vec{v}_2 - 8 \vec{S}_1 \times \vec{v}_1 \cdot \vec{v}_2 \hat{n} \times \vec{S}_1 \cdot \vec{a}_1 - 8 \vec{S}_1 \cdot \vec{a}_1 \hat{n} \cdot \vec{v}_2 \vec{S}_1 \cdot \vec{v}_1 + 8 \vec{S}_1 \cdot \vec{S}_1 \right. \right. \\
& \left. \left. \vec{v}_1 \cdot \vec{a}_1 \hat{n} \cdot \vec{v}_2 + 16 \vec{S}_1 \times \vec{v}_1 \cdot \vec{v}_2 \hat{n} \times \vec{S}_1 \cdot \vec{v}_1 - 8 \vec{S}_1 \times \vec{v}_1 \cdot \vec{v}_2 \hat{n} \times \vec{S}_1 \cdot \vec{v}_1 - 8 \hat{n} \cdot \vec{v}_2 \vec{S}_1 \cdot \vec{v}_1 \vec{S}_1 \cdot \vec{v}_1 + 8 \vec{S}_1 \cdot \vec{S}_1 \vec{v}_1 \cdot \vec{v}_1 \hat{n} \cdot \vec{v}_2 \right) + \right. \\
& \frac{1}{r^4} \left( -16 \vec{v}_1 \cdot \vec{v}_2 \left( \hat{n} \times \vec{S}_1 \cdot \vec{v}_1 \right)^2 + 4 \hat{n} \cdot \vec{v}_1 \hat{n} \cdot \vec{v}_2 \left( \vec{S}_1 \cdot \vec{v}_1 \right)^2 - 4 \vec{v}_1 \cdot \vec{v}_1 \hat{n} \cdot \vec{S}_1 \hat{n} \cdot \vec{v}_2 \vec{S}_1 \cdot \vec{v}_1 + \right. \\
& 4 \vec{S}_1 \cdot \vec{S}_1 \vec{v}_2 \cdot \vec{v}_2 \hat{n} \cdot \vec{v}_1 \hat{n} \cdot \vec{v}_2 - 4 \vec{v}_2 \cdot \vec{v}_2 \hat{n} \cdot \vec{S}_1 \hat{n} \cdot \vec{v}_2 \vec{S}_1 \cdot \vec{v}_1 + 2 \vec{v}_1 \cdot \vec{v}_1 \vec{S}_1 \cdot \vec{v}_1 \vec{S}_1 \cdot \vec{v}_2 - \\
& \left. \left. 2 \vec{v}_1 \cdot \vec{v}_2 \left( \vec{S}_1 \cdot \vec{v}_1 \right)^2 + 2 \vec{v}_2 \cdot \vec{v}_2 \vec{S}_1 \cdot \vec{v}_1 \vec{S}_1 \cdot \vec{v}_2 - 2 \vec{S}_1 \cdot \vec{S}_1 \vec{v}_1 \cdot \vec{v}_2 \vec{v}_2 \cdot \vec{v}_2 \right) \right) \Big\}
\end{aligned}$$

{DiagS1S1[2, 2, 39],

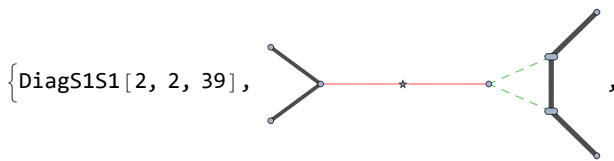

$$\begin{aligned}
& G^2 \left( \frac{1}{r^2} \left( 2 \hat{n} \cdot \vec{v}_1 \hat{n} \cdot \vec{v}_2 \vec{S}_1 \cdot \vec{S}_1 - \vec{v}_1 \cdot \vec{v}_2 \vec{S}_1 \cdot \vec{S}_1 - 2 \hat{n} \cdot \vec{S}_1 \hat{n} \cdot \vec{v}_2 \vec{S}_1 \cdot \vec{a}_1 - 2 \hat{n} \cdot \vec{S}_1 \hat{n} \cdot \vec{v}_2 \vec{S}_1 \cdot \vec{v}_1 + \right. \right. \\
& \frac{1}{\vec{S}_1 \cdot \vec{v}_1 \vec{S}_1 \cdot \vec{v}_2} - 2 \hat{n} \cdot \vec{S}_1 \hat{n} \cdot \vec{v}_2 \vec{S}_1 \cdot \vec{a}_1 + 6 \hat{n} \cdot \vec{a}_1 \hat{n} \cdot \vec{v}_2 \vec{S}_1 \cdot \vec{S}_1 - 3 \vec{a}_1 \cdot \vec{v}_2 \vec{S}_1 \cdot \vec{S}_1 + 2 \hat{n} \cdot \vec{v}_1 \hat{n} \cdot \vec{v}_2 \vec{S}_1 \cdot \vec{S}_1 - \\
& 4 \hat{n} \cdot \vec{S}_1 \hat{n} \cdot \vec{v}_2 \vec{S}_1 \cdot \vec{a}_1 + 2 \vec{S}_1 \cdot \vec{v}_2 \vec{S}_1 \cdot \vec{a}_1 + 2 \hat{n} \cdot \vec{a}_1 \hat{n} \cdot \vec{v}_2 \vec{S}_1 \cdot \vec{S}_1 - \frac{1}{\vec{a}_1 \cdot \vec{v}_2 \vec{S}_1 \cdot \vec{S}_1} - 2 \hat{n} \cdot \vec{S}_1 \hat{n} \cdot \vec{v}_2 \vec{S}_1 \cdot \vec{v}_1 + \\
& \left. \frac{2}{\vec{S}_1 \cdot \vec{v}_2 \vec{S}_1 \cdot \vec{v}_1} + \frac{1}{\vec{S}_1 \cdot \vec{a}_1 \vec{S}_1 \cdot \vec{v}_2} + \vec{S}_1 \cdot \vec{a}_1 \vec{S}_1 \cdot \vec{v}_2 - \vec{S}_1 \cdot \vec{S}_1 \vec{v}_1 \cdot \vec{v}_2 + \frac{3}{2} \hat{n} \cdot \vec{S}_1 \hat{n} \cdot \vec{S}_1 \vec{v}_2 \cdot \vec{a}_2 - \frac{3}{2} \vec{S}_1 \cdot \vec{S}_1 \vec{v}_2 \cdot \vec{a}_2 \right) + \\
& \frac{1}{r^3} \left( -3 \hat{n} \cdot \vec{v}_1 \vec{v}_2 \cdot \vec{a}_2 \left( \hat{n} \cdot \vec{S}_1 \right)^2 + 3 \hat{n} \cdot \vec{v}_1 \hat{n} \cdot \vec{v}_2 \vec{S}_1 \cdot \vec{v}_1 \hat{n} \cdot \vec{S}_1 + 11 \hat{n} \cdot \vec{v}_1 \hat{n} \cdot \vec{v}_2 \vec{S}_1 \cdot \vec{a}_1 \hat{n} \cdot \vec{S}_1 + \right. \\
& 3 \hat{n} \cdot \vec{a}_1 \hat{n} \cdot \vec{v}_2 \vec{S}_1 \cdot \vec{v}_1 \hat{n} \cdot \vec{S}_1 - \frac{3}{4} \vec{a}_1 \cdot \vec{v}_2 \vec{S}_1 \cdot \vec{v}_1 \hat{n} \cdot \vec{S}_1 - \frac{3}{4} \vec{S}_1 \cdot \vec{v}_1 \vec{v}_1 \cdot \vec{v}_2 \hat{n} \cdot \vec{S}_1 - \frac{11}{4} \vec{S}_1 \cdot \vec{a}_1 \vec{v}_1 \cdot \vec{v}_2 \hat{n} \cdot \vec{S}_1 + \\
& \frac{3}{2} \vec{S}_1 \cdot \vec{v}_1 \vec{v}_2 \cdot \vec{a}_2 \hat{n} \cdot \vec{S}_1 + 3 \hat{n} \cdot \vec{S}_1 \hat{n} \cdot \vec{v}_2 \vec{v}_2 \cdot \vec{v}_2 \hat{n} \cdot \vec{S}_1 - \frac{3}{4} \vec{S}_1 \cdot \vec{v}_2 \vec{v}_2 \cdot \vec{v}_2 \hat{n} \cdot \vec{S}_1 - \frac{1}{2} \hat{n} \times \vec{S}_1 \cdot \vec{v}_1 \vec{S}_1 \times \vec{v}_1 \cdot \vec{v}_2 - \\
& \left. \frac{1}{2} \hat{n} \times \vec{S}_1 \cdot \vec{v}_1 \vec{S}_1 \times \vec{a}_1 \cdot \vec{v}_2 - \frac{1}{2} \hat{n} \times \vec{S}_1 \cdot \vec{v}_1 \vec{S}_1 \times \vec{v}_1 \cdot \vec{v}_2 - \frac{1}{2} \hat{n} \times \vec{S}_1 \cdot \vec{a}_1 \vec{S}_1 \times \vec{v}_1 \cdot \vec{v}_2 + 2 \hat{n} \times \vec{S}_1 \cdot \vec{v}_1 \hat{n} \times \vec{S}_1 \cdot \vec{v}_1 \hat{n} \cdot \vec{v}_2 + \right.
\end{aligned}$$

$$\frac{1}{r^4}$$

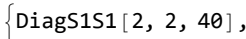

$$\frac{1}{r}$$



$$\begin{aligned}
& 4 \hat{n} \cdot \vec{v}_2 \vec{S}_1 \cdot \vec{S}_1 \vec{v}_1 \cdot \vec{a}_1 - \frac{15}{2} \hat{n} \cdot \vec{v}_1 \vec{S}_1 \cdot \vec{S}_1 \vec{v}_1 \cdot \vec{v}_1 + 4 \hat{n} \cdot \vec{v}_2 \vec{S}_1 \cdot \vec{S}_1 \vec{v}_1 \cdot \vec{v}_1 - 5 \hat{n} \cdot \vec{a}_1 \vec{S}_1 \cdot \vec{S}_1 \vec{v}_1 \cdot \vec{v}_1 \Big) + \frac{1}{r^4} \\
& \left( -24 (\hat{n} \cdot \vec{v}_1)^2 (\hat{n} \times \vec{S}_1 \cdot \vec{v}_1)^2 + 24 \hat{n} \cdot \vec{v}_1 \hat{n} \cdot \vec{v}_2 (\hat{n} \times \vec{S}_1 \cdot \vec{v}_1)^2 + 4 \vec{v}_1 \cdot \vec{v}_1 (\hat{n} \times \vec{S}_1 \cdot \vec{v}_1)^2 - 4 \vec{v}_1 \cdot \vec{v}_2 (\hat{n} \times \vec{S}_1 \cdot \vec{v}_1)^2 - \right. \\
& 3 \vec{v}_2 \cdot \vec{v}_2 (\hat{n} \times \vec{S}_1 \cdot \vec{v}_1)^2 - 8 \vec{S}_1 \times \vec{v}_1 \cdot \vec{v}_2 \hat{n} \cdot \vec{v}_1 \hat{n} \times \vec{S}_1 \cdot \vec{v}_1 - 5 (\hat{n} \cdot \vec{v}_1)^2 (\vec{S}_1 \cdot \vec{v}_1)^2 + 8 \hat{n} \cdot \vec{v}_1 \hat{n} \cdot \vec{v}_2 (\vec{S}_1 \cdot \vec{v}_1)^2 - \\
& 2 \vec{S}_1 \cdot \vec{S}_1 (\vec{v}_1 \cdot \vec{v}_1)^2 + 2 (\vec{S}_1 \cdot \vec{v}_1)^2 \vec{v}_1 \cdot \vec{v}_1 + 8 (\hat{n} \cdot \vec{v}_1)^2 \vec{S}_1 \cdot \vec{S}_1 \vec{v}_1 \cdot \vec{v}_1 - 8 \hat{n} \cdot \vec{v}_1 \hat{n} \cdot \vec{v}_2 \vec{S}_1 \cdot \vec{S}_1 \vec{v}_1 \cdot \vec{v}_1 - \\
& 3 \hat{n} \cdot \vec{S}_1 \hat{n} \cdot \vec{v}_1 \vec{S}_1 \cdot \vec{v}_1 \vec{v}_1 \cdot \vec{v}_1 - 2 (\vec{S}_1 \cdot \vec{v}_1)^2 \vec{v}_1 \cdot \vec{v}_2 + 2 \vec{S}_1 \cdot \vec{S}_1 \vec{v}_1 \cdot \vec{v}_1 \vec{v}_1 \cdot \vec{v}_2 + \frac{3}{2} (\vec{S}_1 \cdot \vec{v}_1)^2 \vec{v}_2 \cdot \vec{v}_2 + \\
& \left. 9 (\hat{n} \cdot \vec{v}_1)^2 \vec{S}_1 \cdot \vec{S}_1 \vec{v}_2 \cdot \vec{v}_2 - 9 \hat{n} \cdot \vec{S}_1 \hat{n} \cdot \vec{v}_1 \vec{S}_1 \cdot \vec{v}_1 \vec{v}_2 \cdot \vec{v}_2 - \frac{3}{2} \vec{S}_1 \cdot \vec{S}_1 \vec{v}_1 \cdot \vec{v}_1 \vec{v}_2 \cdot \vec{v}_2 \right) \Big) m_2 \Big\}
\end{aligned}$$

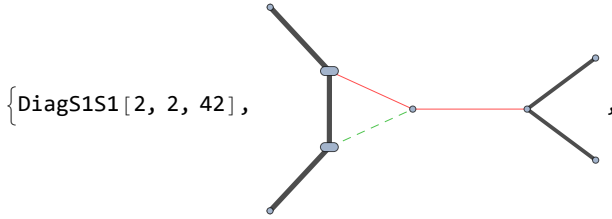

$$\begin{aligned}
& G^2 \left( \frac{1}{r^2} \left( 8 (\hat{n} \times \vec{S}_1 \cdot \vec{v}_1)^2 + 16 \hat{n} \times \vec{S}_1 \cdot \vec{a}_1 \hat{n} \times \vec{S}_1 \cdot \vec{v}_1 + 8 (\hat{n} \times \vec{S}_1 \cdot \vec{a}_1)^2 + 4 (\vec{S}_1 \cdot \vec{v}_1)^2 + \right. \right. \\
& 4 (\vec{S}_1 \cdot \vec{a}_1)^2 - 4 \vec{a}_1 \cdot \vec{a}_1 \vec{S}_1 \cdot \vec{S}_1 + 8 \vec{S}_1 \cdot \vec{a}_1 \vec{S}_1 \cdot \vec{v}_1 - 8 \vec{S}_1 \cdot \vec{S}_1 \vec{v}_1 \cdot \vec{a}_1 - 4 \vec{S}_1 \cdot \vec{S}_1 \vec{v}_1 \cdot \vec{v}_1 \Big) + \frac{1}{r^3} \\
& \left( 6 \hat{n} \times \vec{S}_1 \cdot \vec{v}_1 \vec{S}_1 \times \vec{v}_1 \cdot \vec{v}_2 + 6 \hat{n} \times \vec{S}_1 \cdot \vec{v}_1 \vec{S}_1 \times \vec{a}_1 \cdot \vec{v}_2 - \frac{15}{2} \hat{n} \times \vec{S}_1 \cdot \vec{v}_1 \vec{S}_1 \times \vec{v}_1 \cdot \vec{a}_1 + 6 \hat{n} \times \vec{S}_1 \cdot \vec{v}_1 \vec{S}_1 \times \vec{v}_1 \cdot \vec{v}_2 + \right. \\
& 6 \hat{n} \times \vec{S}_1 \cdot \vec{a}_1 \vec{S}_1 \times \vec{v}_1 \cdot \vec{v}_2 - 32 \hat{n} \times \vec{S}_1 \cdot \vec{v}_1 \hat{n} \times \vec{S}_1 \cdot \vec{v}_1 \hat{n} \cdot \vec{v}_1 - 32 \hat{n} \times \vec{S}_1 \cdot \vec{a}_1 \hat{n} \times \vec{S}_1 \cdot \vec{v}_1 \hat{n} \cdot \vec{v}_1 - \\
& 24 \hat{n} \times \vec{S}_1 \cdot \vec{v}_1 \hat{n} \times \vec{S}_1 \cdot \vec{v}_1 \hat{n} \cdot \vec{v}_2 - 24 \hat{n} \times \vec{S}_1 \cdot \vec{a}_1 \hat{n} \times \vec{S}_1 \cdot \vec{v}_1 \hat{n} \cdot \vec{v}_2 - \frac{19}{2} \hat{n} \cdot \vec{v}_1 \vec{S}_1 \cdot \vec{v}_1 \vec{S}_1 \cdot \vec{v}_1 - 4 \hat{n} \cdot \vec{v}_2 \vec{S}_1 \cdot \vec{v}_1 \vec{S}_1 \cdot \vec{v}_1 - \\
& \frac{19}{2} \hat{n} \cdot \vec{v}_1 \vec{S}_1 \cdot \vec{a}_1 \vec{S}_1 \cdot \vec{v}_1 - 4 \hat{n} \cdot \vec{v}_2 \vec{S}_1 \cdot \vec{a}_1 \vec{S}_1 \cdot \vec{v}_1 + \frac{21}{2} \hat{n} \cdot \vec{v}_1 \vec{S}_1 \cdot \vec{S}_1 \vec{v}_1 \cdot \vec{a}_1 + 4 \hat{n} \cdot \vec{v}_2 \vec{S}_1 \cdot \vec{S}_1 \vec{v}_1 \cdot \vec{a}_1 - \\
& \hat{n} \cdot \vec{S}_1 \vec{S}_1 \cdot \vec{v}_1 \vec{v}_1 \cdot \vec{a}_1 + 10 \hat{n} \cdot \vec{v}_1 \vec{S}_1 \cdot \vec{S}_1 \vec{v}_1 \cdot \vec{v}_1 + 4 \hat{n} \cdot \vec{v}_2 \vec{S}_1 \cdot \vec{S}_1 \vec{v}_1 \cdot \vec{v}_1 - \frac{1}{2} \hat{n} \cdot \vec{S}_1 \vec{S}_1 \cdot \vec{a}_1 \vec{v}_1 \cdot \vec{v}_1 + \\
& \frac{1}{2} \hat{n} \cdot \vec{a}_1 \vec{S}_1 \cdot \vec{S}_1 \vec{v}_1 \cdot \vec{v}_1 - \frac{1}{2} \hat{n} \cdot \vec{S}_1 \vec{S}_1 \cdot \vec{v}_1 \vec{v}_1 \cdot \vec{v}_1 - 3 \hat{n} \cdot \vec{v}_1 \vec{S}_1 \cdot \vec{S}_1 \vec{v}_2 \cdot \vec{a}_2 + 3 \hat{n} \cdot \vec{S}_1 \vec{S}_1 \cdot \vec{v}_1 \vec{v}_2 \cdot \vec{a}_2 + \\
& \frac{3}{2} \hat{n} \cdot \vec{v}_1 \vec{S}_1 \cdot \vec{S}_1 \vec{v}_2 \cdot \vec{v}_2 - \frac{3}{2} \hat{n} \cdot \vec{S}_1 \vec{S}_1 \cdot \vec{a}_1 \vec{v}_2 \cdot \vec{v}_2 + \frac{3}{2} \hat{n} \cdot \vec{a}_1 \vec{S}_1 \cdot \vec{S}_1 \vec{v}_2 \cdot \vec{v}_2 - \frac{3}{2} \hat{n} \cdot \vec{S}_1 \vec{S}_1 \cdot \vec{v}_1 \vec{v}_2 \cdot \vec{v}_2 \Big) + \frac{1}{r^4} \\
& \left( 24 (\hat{n} \cdot \vec{v}_1)^2 (\hat{n} \times \vec{S}_1 \cdot \vec{v}_1)^2 + 24 \hat{n} \cdot \vec{v}_1 \hat{n} \cdot \vec{v}_2 (\hat{n} \times \vec{S}_1 \cdot \vec{v}_1)^2 - 4 \vec{v}_1 \cdot \vec{v}_1 (\hat{n} \times \vec{S}_1 \cdot \vec{v}_1)^2 - 4 \vec{v}_1 \cdot \vec{v}_2 (\hat{n} \times \vec{S}_1 \cdot \vec{v}_1)^2 + \right. \\
& 3 \vec{v}_2 \cdot \vec{v}_2 (\hat{n} \times \vec{S}_1 \cdot \vec{v}_1)^2 - 8 \vec{S}_1 \times \vec{v}_1 \cdot \vec{v}_2 \hat{n} \cdot \vec{v}_1 \hat{n} \times \vec{S}_1 \cdot \vec{v}_1 + 7 (\hat{n} \cdot \vec{v}_1)^2 (\vec{S}_1 \cdot \vec{v}_1)^2 + 6 \hat{n} \cdot \vec{v}_1 \hat{n} \cdot \vec{v}_2 (\vec{S}_1 \cdot \vec{v}_1)^2 + \\
& 2 \vec{S}_1 \cdot \vec{S}_1 (\vec{v}_1 \cdot \vec{v}_1)^2 - 2 (\vec{S}_1 \cdot \vec{v}_1)^2 \vec{v}_1 \cdot \vec{v}_1 - 8 (\hat{n} \cdot \vec{v}_1)^2 \vec{S}_1 \cdot \vec{S}_1 \vec{v}_1 \cdot \vec{v}_1 - 8 \hat{n} \cdot \vec{v}_1 \hat{n} \cdot \vec{v}_2 \vec{S}_1 \cdot \vec{S}_1 \vec{v}_1 \cdot \vec{v}_1 + \\
& \hat{n} \cdot \vec{S}_1 \hat{n} \cdot \vec{v}_1 \vec{S}_1 \cdot \vec{v}_1 \vec{v}_1 \cdot \vec{v}_1 + 2 \hat{n} \cdot \vec{S}_1 \hat{n} \cdot \vec{v}_2 \vec{S}_1 \cdot \vec{v}_1 \vec{v}_1 \cdot \vec{v}_1 - \frac{1}{2} \vec{S}_1 \cdot \vec{v}_1 \vec{S}_1 \cdot \vec{v}_2 \vec{v}_1 \cdot \vec{v}_1 - \frac{3}{2} (\vec{S}_1 \cdot \vec{v}_1)^2 \vec{v}_1 \cdot \vec{v}_2 + \\
& 2 \vec{S}_1 \cdot \vec{S}_1 \vec{v}_1 \cdot \vec{v}_1 \vec{v}_1 \cdot \vec{v}_2 - 3 (\hat{n} \cdot \vec{v}_1)^2 \vec{S}_1 \cdot \vec{S}_1 \vec{v}_2 \cdot \vec{v}_2 - 6 \hat{n} \cdot \vec{v}_1 \hat{n} \cdot \vec{v}_2 \vec{S}_1 \cdot \vec{S}_1 \vec{v}_2 \cdot \vec{v}_2 + 3 \hat{n} \cdot \vec{S}_1 \hat{n} \cdot \vec{v}_1 \vec{S}_1 \cdot \vec{v}_1 \vec{v}_2 \cdot \vec{v}_2 + \\
& \left. 6 \hat{n} \cdot \vec{S}_1 \hat{n} \cdot \vec{v}_2 \vec{S}_1 \cdot \vec{v}_1 \vec{v}_2 \cdot \vec{v}_2 - \frac{3}{2} \vec{S}_1 \cdot \vec{v}_1 \vec{S}_1 \cdot \vec{v}_2 \vec{v}_2 \cdot \vec{v}_2 + \frac{3}{2} \vec{S}_1 \cdot \vec{S}_1 \vec{v}_1 \cdot \vec{v}_2 \vec{v}_2 \cdot \vec{v}_2 \right) \Big) m_2 \Big\}
\end{aligned}$$

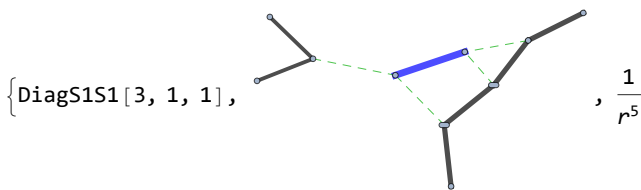

$$G^3 m_1 m_2 \left( \frac{36}{7} \hat{n} \times \vec{S}_1 \cdot \vec{v}_1 \hat{n} \times \vec{S}_1 \cdot \vec{v}_2 - \frac{4}{7} \vec{v}_1 \cdot \vec{v}_2 \left( \hat{n} \cdot \vec{S}_1 \right)^2 + \frac{8}{7} \hat{n} \cdot \vec{S}_1 \hat{n} \cdot \vec{v}_2 \vec{S}_1 \cdot \vec{v}_1 + \right. \\ \left. \frac{16}{7} \hat{n} \cdot \vec{S}_1 \hat{n} \cdot \vec{v}_1 \vec{S}_1 \cdot \vec{v}_2 - \frac{24}{7} \vec{S}_1 \cdot \vec{S}_1 \hat{n} \cdot \vec{v}_1 \hat{n} \cdot \vec{v}_2 + \frac{4}{7} \vec{S}_1 \cdot \vec{v}_1 \vec{S}_1 \cdot \vec{v}_2 - \frac{32}{35} \vec{S}_1 \cdot \vec{S}_1 \vec{v}_1 \cdot \vec{v}_2 \right) \Bigg\}$$

{DiagS1S1[3, 1, 2],

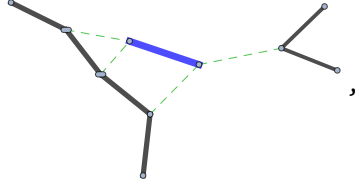

$$G^3 m_1 m_2 \left( \frac{1}{r^5 \in_d} \left( -4 \left( \hat{n} \cdot \vec{S}_1 \right)^2 \hat{n} \cdot \vec{v}_1 \hat{n} \cdot \vec{v}_2 + \frac{4}{7} \vec{v}_1 \cdot \vec{v}_2 \left( \hat{n} \cdot \vec{S}_1 \right)^2 + \frac{8}{7} \hat{n} \cdot \vec{S}_1 \hat{n} \cdot \vec{v}_2 \vec{S}_1 \cdot \vec{v}_1 + \right. \right. \\ \left. \frac{8}{7} \hat{n} \cdot \vec{S}_1 \hat{n} \cdot \vec{v}_1 \vec{S}_1 \cdot \vec{v}_2 + \frac{4}{7} \vec{S}_1 \cdot \vec{S}_1 \hat{n} \cdot \vec{v}_1 \hat{n} \cdot \vec{v}_2 - \frac{8}{35} \vec{S}_1 \cdot \vec{v}_1 \vec{S}_1 \cdot \vec{v}_2 - \frac{4}{35} \vec{S}_1 \cdot \vec{S}_1 \vec{v}_1 \cdot \vec{v}_2 \right) + \\ \frac{1}{r^5} \log \left( \frac{r}{R_0} \right) \left( 12 \left( \hat{n} \cdot \vec{S}_1 \right)^2 \hat{n} \cdot \vec{v}_1 \hat{n} \cdot \vec{v}_2 - \frac{12}{7} \vec{v}_1 \cdot \vec{v}_2 \left( \hat{n} \cdot \vec{S}_1 \right)^2 - \frac{24}{7} \hat{n} \cdot \vec{S}_1 \hat{n} \cdot \vec{v}_2 \vec{S}_1 \cdot \vec{v}_1 - \right. \\ \left. \frac{24}{7} \hat{n} \cdot \vec{S}_1 \hat{n} \cdot \vec{v}_1 \vec{S}_1 \cdot \vec{v}_2 - \frac{12}{7} \vec{S}_1 \cdot \vec{S}_1 \hat{n} \cdot \vec{v}_1 \hat{n} \cdot \vec{v}_2 + \frac{24}{35} \vec{S}_1 \cdot \vec{v}_1 \vec{S}_1 \cdot \vec{v}_2 + \frac{12}{35} \vec{S}_1 \cdot \vec{S}_1 \vec{v}_1 \cdot \vec{v}_2 \right) + \frac{1}{r^5} \\ \left. \left( \frac{16}{7} \hat{n} \times \vec{S}_1 \cdot \vec{v}_1 \hat{n} \times \vec{S}_1 \cdot \vec{v}_2 - \frac{55}{3} \left( \hat{n} \cdot \vec{S}_1 \right)^2 \hat{n} \cdot \vec{v}_1 \hat{n} \cdot \vec{v}_2 + \frac{643}{147} \vec{v}_1 \cdot \vec{v}_2 \left( \hat{n} \cdot \vec{S}_1 \right)^2 + \frac{362}{147} \hat{n} \cdot \vec{S}_1 \hat{n} \cdot \vec{v}_2 \vec{S}_1 \cdot \vec{v}_1 + \right. \right. \\ \left. \left. \frac{362}{147} \hat{n} \cdot \vec{S}_1 \hat{n} \cdot \vec{v}_1 \vec{S}_1 \cdot \vec{v}_2 + \frac{937}{147} \vec{S}_1 \cdot \vec{S}_1 \hat{n} \cdot \vec{v}_1 \hat{n} \cdot \vec{v}_2 + \frac{5834 \vec{S}_1 \cdot \vec{v}_1 \vec{S}_1 \cdot \vec{v}_2}{3675} - \frac{9683 \vec{S}_1 \cdot \vec{S}_1 \vec{v}_1 \cdot \vec{v}_2}{3675} \right) \right) \Bigg\}$$

{DiagS1S1[3, 1, 3],

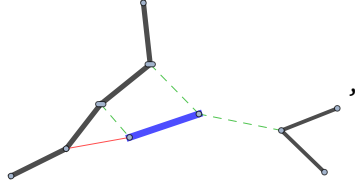

$$G^3 m_1 m_2 \left( \frac{2 \hat{n} \cdot \vec{S}_1 \hat{n} \cdot \vec{S}_1 \hat{n} \cdot \vec{v}_2 - \frac{2}{5} \vec{S}_1 \cdot \vec{S}_1 \hat{n} \cdot \vec{v}_2 - \frac{2}{5} \hat{n} \cdot \vec{S}_1 \vec{S}_1 \cdot \vec{v}_2 - \frac{1}{5} \hat{n} \cdot \vec{S}_1 \vec{S}_1 \cdot \vec{v}_2}{r^4 \in_d} + \right. \\ \left. \frac{-6 \hat{n} \times \vec{S}_1 \cdot \vec{v}_1 \hat{n} \times \vec{S}_1 \cdot \vec{v}_2 + 2 \vec{S}_1 \cdot \vec{S}_1 \hat{n} \cdot \vec{v}_1 \hat{n} \cdot \vec{v}_2 - 2 \hat{n} \cdot \vec{S}_1 \hat{n} \cdot \vec{v}_2 \vec{S}_1 \cdot \vec{v}_1 - \frac{12}{5} \vec{S}_1 \cdot \vec{v}_1 \vec{S}_1 \cdot \vec{v}_2 + \frac{12}{5} \vec{S}_1 \cdot \vec{S}_1 \vec{v}_1 \cdot \vec{v}_2}{r^5} + \right. \\ \left. \frac{\log \left( \frac{r}{R_0} \right) \left( -6 \hat{n} \cdot \vec{S}_1 \hat{n} \cdot \vec{S}_1 \hat{n} \cdot \vec{v}_2 + \frac{6}{5} \vec{S}_1 \cdot \vec{S}_1 \hat{n} \cdot \vec{v}_2 + \frac{6}{5} \hat{n} \cdot \vec{S}_1 \vec{S}_1 \cdot \vec{v}_2 + \frac{6}{5} \hat{n} \cdot \vec{S}_1 \vec{S}_1 \cdot \vec{v}_2 \right)}{r^4} + \right. \\ \left. \frac{9 \hat{n} \cdot \vec{S}_1 \hat{n} \cdot \vec{S}_1 \hat{n} \cdot \vec{v}_2 - \frac{169}{25} \vec{S}_1 \cdot \vec{S}_1 \hat{n} \cdot \vec{v}_2 + \frac{31}{25} \hat{n} \cdot \vec{S}_1 \vec{S}_1 \cdot \vec{v}_2 - \frac{69}{25} \hat{n} \cdot \vec{S}_1 \vec{S}_1 \cdot \vec{v}_2}{r^4} \right) \Bigg\}$$

{DiagS1S1[3, 1, 4],

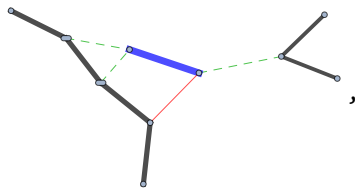

$$\begin{aligned}
& G^3 m_1 m_2 \left( \frac{-\frac{164}{49} \hat{n} \cdot \vec{a}_2 \left( \hat{n} \cdot \vec{S}_1 \right)^2 + \frac{1458 \vec{S}_1 \cdot \vec{a}_2 \hat{n} \cdot \vec{S}_1}{1225} + \frac{1184 \hat{n} \cdot \vec{a}_2 \vec{S}_1 \cdot \vec{S}_1}{1225}}{r^4} + \frac{1}{r^5} \right. \\
& \left( -26 \left( \hat{n} \cdot \vec{v}_2 \right)^2 \left( \hat{n} \cdot \vec{S}_1 \right)^2 + \frac{55}{12} \hat{n} \cdot \vec{v}_1 \hat{n} \cdot \vec{v}_2 \left( \hat{n} \cdot \vec{S}_1 \right)^2 + \frac{155}{588} \vec{v}_1 \cdot \vec{v}_2 \left( \hat{n} \cdot \vec{S}_1 \right)^2 + \frac{164}{49} \vec{v}_2 \cdot \vec{v}_2 \left( \hat{n} \cdot \vec{S}_1 \right)^2 - \right. \\
& \frac{349}{294} \hat{n} \cdot \vec{v}_2 \vec{S}_1 \cdot \vec{v}_1 \hat{n} \cdot \vec{S}_1 - \frac{601}{294} \hat{n} \cdot \vec{v}_1 \vec{S}_1 \cdot \vec{v}_2 \hat{n} \cdot \vec{S}_1 + \frac{670}{49} \hat{n} \cdot \vec{v}_2 \vec{S}_1 \cdot \vec{v}_2 \hat{n} \cdot \vec{S}_1 - \frac{1458 \left( \vec{S}_1 \cdot \vec{v}_2 \right)^2}{1225} + \\
& \frac{4}{7} \hat{n} \times \vec{S}_1 \cdot \vec{v}_1 \hat{n} \times \vec{S}_1 \cdot \vec{v}_2 + \frac{262}{49} \left( \hat{n} \cdot \vec{v}_2 \right)^2 \vec{S}_1 \cdot \vec{S}_1 - \frac{265}{588} \hat{n} \cdot \vec{v}_1 \hat{n} \cdot \vec{v}_2 \vec{S}_1 \cdot \vec{S}_1 + \frac{5273 \vec{S}_1 \cdot \vec{v}_1 \vec{S}_1 \cdot \vec{v}_2}{7350} - \\
& \left. \frac{8167 \vec{S}_1 \cdot \vec{S}_1 \vec{v}_1 \cdot \vec{v}_2}{14700} - \frac{1184 \vec{S}_1 \cdot \vec{S}_1 \vec{v}_2 \cdot \vec{v}_2}{1225} \right) + \left( \frac{\frac{18}{7} \hat{n} \cdot \vec{a}_2 \left( \hat{n} \cdot \vec{S}_1 \right)^2 - \frac{36}{35} \vec{S}_1 \cdot \vec{a}_2 \hat{n} \cdot \vec{S}_1 - \frac{18}{35} \hat{n} \cdot \vec{a}_2 \vec{S}_1 \cdot \vec{S}_1}{r^4} + \right. \\
& \frac{1}{r^5} \left( 18 \left( \hat{n} \cdot \vec{v}_2 \right)^2 \left( \hat{n} \cdot \vec{S}_1 \right)^2 - 3 \hat{n} \cdot \vec{v}_1 \hat{n} \cdot \vec{v}_2 \left( \hat{n} \cdot \vec{S}_1 \right)^2 + \frac{3}{7} \vec{v}_1 \cdot \vec{v}_2 \left( \hat{n} \cdot \vec{S}_1 \right)^2 - \frac{18}{7} \vec{v}_2 \cdot \vec{v}_2 \left( \hat{n} \cdot \vec{S}_1 \right)^2 + \right. \\
& \frac{6}{7} \hat{n} \cdot \vec{v}_2 \vec{S}_1 \cdot \vec{v}_1 \hat{n} \cdot \vec{S}_1 + \frac{6}{7} \hat{n} \cdot \vec{v}_1 \vec{S}_1 \cdot \vec{v}_2 \hat{n} \cdot \vec{S}_1 - \frac{72}{7} \hat{n} \cdot \vec{v}_2 \vec{S}_1 \cdot \vec{v}_2 \hat{n} \cdot \vec{S}_1 + \frac{36}{35} \left( \vec{S}_1 \cdot \vec{v}_2 \right)^2 - \\
& \left. \frac{18}{7} \left( \hat{n} \cdot \vec{v}_2 \right)^2 \vec{S}_1 \cdot \vec{S}_1 + \frac{3}{7} \hat{n} \cdot \vec{v}_1 \hat{n} \cdot \vec{v}_2 \vec{S}_1 \cdot \vec{S}_1 - \frac{6}{35} \vec{S}_1 \cdot \vec{v}_1 \vec{S}_1 \cdot \vec{v}_2 - \frac{3}{35} \vec{S}_1 \cdot \vec{S}_1 \vec{v}_1 \cdot \vec{v}_2 + \frac{18}{35} \vec{S}_1 \cdot \vec{S}_1 \vec{v}_2 \cdot \vec{v}_2 \right) \left. \right) \\
& \log \left( \frac{r}{R_0} \right) + \frac{1}{\epsilon_d} \left( \frac{-\frac{6}{7} \hat{n} \cdot \vec{a}_2 \left( \hat{n} \cdot \vec{S}_1 \right)^2 + \frac{12}{35} \vec{S}_1 \cdot \vec{a}_2 \hat{n} \cdot \vec{S}_1 + \frac{6}{35} \hat{n} \cdot \vec{a}_2 \vec{S}_1 \cdot \vec{S}_1}{r^4} + \frac{1}{r^5} \right. \\
& \left( -6 \left( \hat{n} \cdot \vec{v}_2 \right)^2 \left( \hat{n} \cdot \vec{S}_1 \right)^2 + \hat{n} \cdot \vec{v}_1 \hat{n} \cdot \vec{v}_2 \left( \hat{n} \cdot \vec{S}_1 \right)^2 - \frac{1}{7} \vec{v}_1 \cdot \vec{v}_2 \left( \hat{n} \cdot \vec{S}_1 \right)^2 + \frac{6}{7} \vec{v}_2 \cdot \vec{v}_2 \left( \hat{n} \cdot \vec{S}_1 \right)^2 - \right. \\
& \frac{2}{7} \hat{n} \cdot \vec{v}_2 \vec{S}_1 \cdot \vec{v}_1 \hat{n} \cdot \vec{S}_1 - \frac{2}{7} \hat{n} \cdot \vec{v}_1 \vec{S}_1 \cdot \vec{v}_2 \hat{n} \cdot \vec{S}_1 + \frac{24}{7} \hat{n} \cdot \vec{v}_2 \vec{S}_1 \cdot \vec{v}_2 \hat{n} \cdot \vec{S}_1 - \frac{12}{35} \left( \vec{S}_1 \cdot \vec{v}_2 \right)^2 + \\
& \left. \frac{6}{7} \left( \hat{n} \cdot \vec{v}_2 \right)^2 \vec{S}_1 \cdot \vec{S}_1 - \frac{1}{7} \hat{n} \cdot \vec{v}_1 \hat{n} \cdot \vec{v}_2 \vec{S}_1 \cdot \vec{S}_1 + \frac{2}{35} \vec{S}_1 \cdot \vec{v}_1 \vec{S}_1 \cdot \vec{v}_2 + \frac{1}{35} \vec{S}_1 \cdot \vec{S}_1 \vec{v}_1 \cdot \vec{v}_2 - \frac{6}{35} \vec{S}_1 \cdot \vec{S}_1 \vec{v}_2 \cdot \vec{v}_2 \right) \left. \right) \left. \right) \Bigg\}
\end{aligned}$$

{DiagS1S1[3, 1, 5],

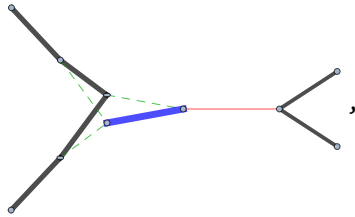

$$\begin{aligned}
& G^3 m_1 m_2 \left( \frac{-5 \hat{n} \cdot \vec{S}_1 \hat{n} \cdot \vec{S}_1 \hat{n} \cdot \vec{v}_1 + \frac{89}{25} \vec{S}_1 \cdot \vec{S}_1 \hat{n} \cdot \vec{v}_1 + \frac{9}{25} \hat{n} \cdot \vec{S}_1 \vec{S}_1 \cdot \vec{v}_1 + \frac{9}{25} \hat{n} \cdot \vec{S}_1 \vec{S}_1 \cdot \vec{v}_1}{r^4} + \frac{1}{r^5} \right. \\
& \left( \frac{30}{7} \left( \hat{n} \times \vec{S}_1 \cdot \vec{v}_1 \right)^2 + 17 \left( \hat{n} \cdot \vec{S}_1 \right)^2 \left( \hat{n} \cdot \vec{v}_1 \right)^2 + \frac{898 \left( \vec{S}_1 \cdot \vec{v}_1 \right)^2}{1225} - 17 \left( \hat{n} \cdot \vec{S}_1 \right)^2 \hat{n} \cdot \vec{v}_1 \hat{n} \cdot \vec{v}_2 - \frac{381}{49} \left( \hat{n} \cdot \vec{v}_1 \right)^2 \vec{S}_1 \cdot \vec{S}_1 + \right. \\
& \frac{395}{49} \hat{n} \cdot \vec{v}_1 \hat{n} \cdot \vec{v}_2 \vec{S}_1 \cdot \vec{S}_1 - \frac{334}{49} \hat{n} \cdot \vec{S}_1 \hat{n} \cdot \vec{v}_1 \vec{S}_1 \cdot \vec{v}_1 + \frac{118}{49} \hat{n} \cdot \vec{S}_1 \hat{n} \cdot \vec{v}_2 \vec{S}_1 \cdot \vec{v}_1 + \frac{202}{49} \hat{n} \cdot \vec{S}_1 \hat{n} \cdot \vec{v}_1 \vec{S}_1 \cdot \vec{v}_2 - \\
& \left. \frac{338 \vec{S}_1 \cdot \vec{v}_1 \vec{S}_1 \cdot \vec{v}_2}{1225} - \frac{101}{49} \left( \hat{n} \cdot \vec{S}_1 \right)^2 \vec{v}_1 \cdot \vec{v}_1 + \frac{1289 \vec{S}_1 \cdot \vec{S}_1 \vec{v}_1 \cdot \vec{v}_1}{1225} + \frac{101}{49} \left( \hat{n} \cdot \vec{S}_1 \right)^2 \vec{v}_1 \cdot \vec{v}_2 - \frac{1849 \vec{S}_1 \cdot \vec{S}_1 \vec{v}_1 \cdot \vec{v}_2}{1225} \right) + \left. \right)
\end{aligned}$$

$$\begin{aligned}
& \left( \frac{6 \hat{n} \cdot \vec{S}_1 \hat{n} \cdot \vec{S}_1 \hat{n} \cdot \vec{v}_1 - \frac{6}{5} \vec{S}_1 \cdot \vec{S}_1 \hat{n} \cdot \vec{v}_1 - \frac{6}{5} \hat{n} \cdot \vec{S}_1 \vec{S}_1 \cdot \vec{v}_1 - \frac{6}{5} \hat{n} \cdot \vec{S}_1 \vec{S}_1 \cdot \vec{v}_1}{r^4} + \frac{1}{r^5} \right. \\
& \left( -18 (\hat{n} \cdot \vec{v}_1)^2 (\hat{n} \cdot \vec{S}_1)^2 + 18 \hat{n} \cdot \vec{v}_1 \hat{n} \cdot \vec{v}_2 (\hat{n} \cdot \vec{S}_1)^2 + \frac{18}{7} \vec{v}_1 \cdot \vec{v}_1 (\hat{n} \cdot \vec{S}_1)^2 - \frac{18}{7} \vec{v}_1 \cdot \vec{v}_2 (\hat{n} \cdot \vec{S}_1)^2 + \right. \\
& \frac{72}{7} \hat{n} \cdot \vec{v}_1 \vec{S}_1 \cdot \vec{v}_1 \hat{n} \cdot \vec{S}_1 - \frac{36}{7} \hat{n} \cdot \vec{v}_2 \vec{S}_1 \cdot \vec{v}_1 \hat{n} \cdot \vec{S}_1 - \frac{36}{7} \hat{n} \cdot \vec{v}_1 \vec{S}_1 \cdot \vec{v}_2 \hat{n} \cdot \vec{S}_1 - \frac{36}{35} (\vec{S}_1 \cdot \vec{v}_1)^2 + \frac{18}{7} (\hat{n} \cdot \vec{v}_1)^2 \vec{S}_1 \cdot \vec{S}_1 - \\
& \left. \frac{18}{7} \hat{n} \cdot \vec{v}_1 \hat{n} \cdot \vec{v}_2 \vec{S}_1 \cdot \vec{S}_1 + \frac{36}{35} \vec{S}_1 \cdot \vec{v}_1 \vec{S}_1 \cdot \vec{v}_2 - \frac{18}{35} \vec{S}_1 \cdot \vec{S}_1 \vec{v}_1 \cdot \vec{v}_1 + \frac{18}{35} \vec{S}_1 \cdot \vec{S}_1 \vec{v}_1 \cdot \vec{v}_2 \right) \log \left( \frac{r}{R_\theta} \right) + \\
& \frac{1}{\epsilon_d} \left( \frac{-2 \hat{n} \cdot \vec{S}_1 \hat{n} \cdot \vec{S}_1 \hat{n} \cdot \vec{v}_1 + \frac{2}{5} \vec{S}_1 \cdot \vec{S}_1 \hat{n} \cdot \vec{v}_1 + \frac{2}{5} \hat{n} \cdot \vec{S}_1 \vec{S}_1 \cdot \vec{v}_1 + \frac{2}{5} \hat{n} \cdot \vec{S}_1 \vec{S}_1 \cdot \vec{v}_1}{r^4} + \frac{1}{r^5} \right. \\
& \left( 6 (\hat{n} \cdot \vec{v}_1)^2 (\hat{n} \cdot \vec{S}_1)^2 - 6 \hat{n} \cdot \vec{v}_1 \hat{n} \cdot \vec{v}_2 (\hat{n} \cdot \vec{S}_1)^2 - \frac{6}{7} \vec{v}_1 \cdot \vec{v}_1 (\hat{n} \cdot \vec{S}_1)^2 + \frac{6}{7} \vec{v}_1 \cdot \vec{v}_2 (\hat{n} \cdot \vec{S}_1)^2 - \right. \\
& \frac{24}{7} \hat{n} \cdot \vec{v}_1 \vec{S}_1 \cdot \vec{v}_1 \hat{n} \cdot \vec{S}_1 + \frac{12}{7} \hat{n} \cdot \vec{v}_2 \vec{S}_1 \cdot \vec{v}_1 \hat{n} \cdot \vec{S}_1 + \frac{12}{7} \hat{n} \cdot \vec{v}_1 \vec{S}_1 \cdot \vec{v}_2 \hat{n} \cdot \vec{S}_1 + \frac{12}{35} (\vec{S}_1 \cdot \vec{v}_1)^2 - \\
& \left. \frac{6}{7} (\hat{n} \cdot \vec{v}_1)^2 \vec{S}_1 \cdot \vec{S}_1 + \frac{6}{7} \hat{n} \cdot \vec{v}_1 \hat{n} \cdot \vec{v}_2 \vec{S}_1 \cdot \vec{S}_1 - \frac{12}{35} \vec{S}_1 \cdot \vec{v}_1 \vec{S}_1 \cdot \vec{v}_2 + \frac{6}{35} \vec{S}_1 \cdot \vec{S}_1 \vec{v}_1 \cdot \vec{v}_1 - \frac{6}{35} \vec{S}_1 \cdot \vec{S}_1 \vec{v}_1 \cdot \vec{v}_2 \right) \left. \right) \Bigg\}
\end{aligned}$$

{DiagS1S1[3, 1, 6],

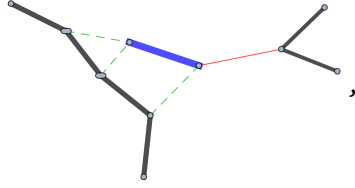

$$\begin{aligned}
& G^3 m_1 m_2 \left( \frac{\frac{164}{49} \hat{n} \cdot \vec{a}_1 (\hat{n} \cdot \vec{S}_1)^2 - \frac{1458 \vec{S}_1 \cdot \vec{a}_1 \hat{n} \cdot \vec{S}_1}{1225} - \frac{1184 \hat{n} \cdot \vec{a}_1 \vec{S}_1 \cdot \vec{S}_1}{1225}}{r^4} + \frac{1}{r^5} \right. \\
& \left( -\frac{4}{7} (\hat{n} \times \vec{S}_1 \cdot \vec{v}_1)^2 - \frac{55}{12} (\hat{n} \cdot \vec{S}_1)^2 (\hat{n} \cdot \vec{v}_1)^2 - \frac{5273 (\vec{S}_1 \cdot \vec{v}_1)^2}{7350} + 26 (\hat{n} \cdot \vec{S}_1)^2 \hat{n} \cdot \vec{v}_1 \hat{n} \cdot \vec{v}_2 + \frac{265}{588} (\hat{n} \cdot \vec{v}_1)^2 \vec{S}_1 \cdot \vec{S}_1 - \right. \\
& \frac{262}{49} \hat{n} \cdot \vec{v}_1 \hat{n} \cdot \vec{v}_2 \vec{S}_1 \cdot \vec{S}_1 + \frac{475}{147} \hat{n} \cdot \vec{S}_1 \hat{n} \cdot \vec{v}_1 \vec{S}_1 \cdot \vec{v}_1 - \frac{342}{49} \hat{n} \cdot \vec{S}_1 \hat{n} \cdot \vec{v}_2 \vec{S}_1 \cdot \vec{v}_1 - \frac{328}{49} \hat{n} \cdot \vec{S}_1 \hat{n} \cdot \vec{v}_1 \vec{S}_1 \cdot \vec{v}_2 + \\
& \left. \frac{1458 \vec{S}_1 \cdot \vec{v}_1 \vec{S}_1 \cdot \vec{v}_2}{1225} - \frac{155}{588} (\hat{n} \cdot \vec{S}_1)^2 \vec{v}_1 \cdot \vec{v}_1 + \frac{8167 \vec{S}_1 \cdot \vec{S}_1 \vec{v}_1 \cdot \vec{v}_1}{14700} - \frac{164}{49} (\hat{n} \cdot \vec{S}_1)^2 \vec{v}_1 \cdot \vec{v}_2 + \frac{1184 \vec{S}_1 \cdot \vec{S}_1 \vec{v}_1 \cdot \vec{v}_2}{1225} \right) + \\
& \left( -\frac{18}{7} \hat{n} \cdot \vec{a}_1 (\hat{n} \cdot \vec{S}_1)^2 + \frac{36}{35} \vec{S}_1 \cdot \vec{a}_1 \hat{n} \cdot \vec{S}_1 + \frac{18}{35} \hat{n} \cdot \vec{a}_1 \vec{S}_1 \cdot \vec{S}_1}{r^4} + \frac{1}{r^5} \right. \\
& \left( 3 (\hat{n} \cdot \vec{v}_1)^2 (\hat{n} \cdot \vec{S}_1)^2 - 18 \hat{n} \cdot \vec{v}_1 \hat{n} \cdot \vec{v}_2 (\hat{n} \cdot \vec{S}_1)^2 - \frac{3}{7} \vec{v}_1 \cdot \vec{v}_1 (\hat{n} \cdot \vec{S}_1)^2 + \frac{18}{7} \vec{v}_1 \cdot \vec{v}_2 (\hat{n} \cdot \vec{S}_1)^2 - \right. \\
& \frac{12}{7} \hat{n} \cdot \vec{v}_1 \vec{S}_1 \cdot \vec{v}_1 \hat{n} \cdot \vec{S}_1 + \frac{36}{7} \hat{n} \cdot \vec{v}_2 \vec{S}_1 \cdot \vec{v}_1 \hat{n} \cdot \vec{S}_1 + \frac{36}{7} \hat{n} \cdot \vec{v}_1 \vec{S}_1 \cdot \vec{v}_2 \hat{n} \cdot \vec{S}_1 + \frac{6}{35} (\vec{S}_1 \cdot \vec{v}_1)^2 - \\
& \left. \frac{3}{7} (\hat{n} \cdot \vec{v}_1)^2 \vec{S}_1 \cdot \vec{S}_1 + \frac{18}{7} \hat{n} \cdot \vec{v}_1 \hat{n} \cdot \vec{v}_2 \vec{S}_1 \cdot \vec{S}_1 - \frac{36}{35} \vec{S}_1 \cdot \vec{v}_1 \vec{S}_1 \cdot \vec{v}_2 + \frac{3}{35} \vec{S}_1 \cdot \vec{S}_1 \vec{v}_1 \cdot \vec{v}_1 - \frac{18}{35} \vec{S}_1 \cdot \vec{S}_1 \vec{v}_1 \cdot \vec{v}_2 \right) \left. \right)
\end{aligned}$$

$$\log\left(\frac{r}{R_\theta}\right) + \frac{1}{\epsilon_d} \left( \frac{\frac{6}{7} \hat{n} \cdot \vec{a}_1 \left( \hat{n} \cdot \vec{S}_1 \right)^2 - \frac{12}{35} \vec{S}_1 \cdot \vec{a}_1 \hat{n} \cdot \vec{S}_1 - \frac{6}{35} \hat{n} \cdot \vec{a}_1 \vec{S}_1 \cdot \vec{S}_1}{r^4} + \frac{1}{r^5} \right. \\ \left. \left( - \left( \hat{n} \cdot \vec{v}_1 \right)^2 \left( \hat{n} \cdot \vec{S}_1 \right)^2 + 6 \hat{n} \cdot \vec{v}_1 \hat{n} \cdot \vec{v}_2 \left( \hat{n} \cdot \vec{S}_1 \right)^2 + \frac{1}{7} \vec{v}_1 \cdot \vec{v}_1 \left( \hat{n} \cdot \vec{S}_1 \right)^2 - \frac{6}{7} \vec{v}_1 \cdot \vec{v}_2 \left( \hat{n} \cdot \vec{S}_1 \right)^2 + \right. \right. \\ \left. \frac{4}{7} \hat{n} \cdot \vec{v}_1 \vec{S}_1 \cdot \vec{v}_1 \hat{n} \cdot \vec{S}_1 - \frac{12}{7} \hat{n} \cdot \vec{v}_2 \vec{S}_1 \cdot \vec{v}_1 \hat{n} \cdot \vec{S}_1 - \frac{12}{7} \hat{n} \cdot \vec{v}_1 \vec{S}_1 \cdot \vec{v}_2 \hat{n} \cdot \vec{S}_1 - \frac{2}{35} \left( \vec{S}_1 \cdot \vec{v}_1 \right)^2 + \right. \\ \left. \left. \frac{1}{7} \left( \hat{n} \cdot \vec{v}_1 \right)^2 \vec{S}_1 \cdot \vec{S}_1 - \frac{6}{7} \hat{n} \cdot \vec{v}_1 \hat{n} \cdot \vec{v}_2 \vec{S}_1 \cdot \vec{S}_1 + \frac{12}{35} \vec{S}_1 \cdot \vec{v}_1 \vec{S}_1 \cdot \vec{v}_2 - \frac{1}{35} \vec{S}_1 \cdot \vec{S}_1 \vec{v}_1 \cdot \vec{v}_1 + \frac{6}{35} \vec{S}_1 \cdot \vec{S}_1 \vec{v}_1 \cdot \vec{v}_2 \right) \right) \right\}$$

{DiagS1S1[3, 1, 7],

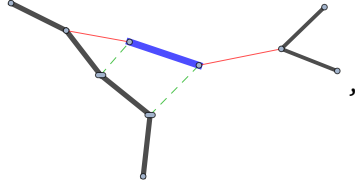

$$G^3 m_1 m_2 \left( \frac{\frac{158}{75} \vec{S}_1 \cdot \vec{S}_1 - \frac{78}{25} \left( \hat{n} \cdot \vec{S}_1 \right)^2}{r^3} + \frac{1}{r^4} \left( \frac{513}{49} \hat{n} \cdot \vec{S}_1 \hat{n} \cdot \vec{S}_1 \hat{n} \cdot \vec{v}_1 - \frac{7577 \vec{S}_1 \cdot \vec{S}_1 \hat{n} \cdot \vec{v}_1}{1225} - 23 \hat{n} \cdot \vec{S}_1 \hat{n} \cdot \vec{S}_1 \hat{n} \cdot \vec{v}_2 - \right. \right.$$

$$\left. \frac{577 \hat{n} \cdot \vec{S}_1 \vec{S}_1 \cdot \vec{v}_1}{1225} + \frac{97}{25} \hat{n} \cdot \vec{S}_1 \vec{S}_1 \cdot \vec{v}_2 + \frac{247}{25} \hat{n} \cdot \vec{v}_2 \vec{S}_1 \cdot \vec{S}_1 - \frac{1557 \hat{n} \cdot \vec{S}_1 \vec{S}_1 \cdot \vec{v}_1}{1225} + \frac{97}{25} \hat{n} \cdot \vec{S}_1 \vec{S}_1 \cdot \vec{v}_2 \right) + \frac{1}{r^5}$$

$$\left( - \frac{6}{7} \left( \hat{n} \times \vec{S}_1 \cdot \vec{v}_1 \right)^2 + \frac{8}{7} \left( \vec{S}_1 \cdot \vec{v}_1 \right)^2 + \frac{30}{7} \left( \hat{n} \cdot \vec{v}_1 \right)^2 \vec{S}_1 \cdot \vec{S}_1 - 6 \hat{n} \cdot \vec{v}_1 \hat{n} \cdot \vec{v}_2 \vec{S}_1 \cdot \vec{S}_1 - \frac{30}{7} \hat{n} \cdot \vec{S}_1 \hat{n} \cdot \vec{v}_1 \vec{S}_1 \cdot \vec{v}_1 + \right. \\ \left. 6 \hat{n} \cdot \vec{S}_1 \hat{n} \cdot \vec{v}_2 \vec{S}_1 \cdot \vec{v}_1 - \frac{6}{5} \vec{S}_1 \cdot \vec{v}_1 \vec{S}_1 \cdot \vec{v}_2 - \frac{8}{7} \vec{S}_1 \cdot \vec{S}_1 \vec{v}_1 \cdot \vec{v}_1 + \frac{6}{5} \vec{S}_1 \cdot \vec{S}_1 \vec{v}_1 \cdot \vec{v}_2 \right) +$$

$$\left( \frac{\frac{12}{5} \left( \hat{n} \cdot \vec{S}_1 \right)^2 - \frac{4}{5} \vec{S}_1 \cdot \vec{S}_1}{r^3} + \frac{1}{r^4} \left( - \frac{54}{7} \hat{n} \cdot \vec{S}_1 \hat{n} \cdot \vec{S}_1 \hat{n} \cdot \vec{v}_1 + \frac{54}{35} \vec{S}_1 \cdot \vec{S}_1 \hat{n} \cdot \vec{v}_1 + 18 \hat{n} \cdot \vec{S}_1 \hat{n} \cdot \vec{S}_1 \hat{n} \cdot \vec{v}_2 + \right. \right.$$

$$\left. \frac{54}{35} \hat{n} \cdot \vec{S}_1 \vec{S}_1 \cdot \vec{v}_1 - \frac{18}{5} \hat{n} \cdot \vec{S}_1 \vec{S}_1 \cdot \vec{v}_2 - \frac{18}{5} \hat{n} \cdot \vec{v}_2 \vec{S}_1 \cdot \vec{S}_1 + \frac{54}{35} \hat{n} \cdot \vec{S}_1 \vec{S}_1 \cdot \vec{v}_1 - \frac{18}{5} \hat{n} \cdot \vec{S}_1 \vec{S}_1 \cdot \vec{v}_2 \right) \log\left(\frac{r}{R_\theta}\right) +$$

$$\left. \frac{\frac{4}{15} \vec{S}_1 \cdot \vec{S}_1 - \frac{4}{5} \left( \hat{n} \cdot \vec{S}_1 \right)^2}{r^3} + \frac{18}{7} \hat{n} \cdot \vec{S}_1 \hat{n} \cdot \vec{S}_1 \hat{n} \cdot \vec{v}_1 - \frac{18}{35} \vec{S}_1 \cdot \vec{S}_1 \hat{n} \cdot \vec{v}_1 - 6 \hat{n} \cdot \vec{S}_1 \hat{n} \cdot \vec{S}_1 \hat{n} \cdot \vec{v}_2 - \frac{18}{35} \hat{n} \cdot \vec{S}_1 \vec{S}_1 \cdot \vec{v}_1 + \frac{6}{5} \hat{n} \cdot \vec{S}_1 \vec{S}_1 \cdot \vec{v}_2 + \frac{6}{5} \hat{n} \cdot \vec{v}_2 \vec{S}_1 \cdot \vec{S}_1 - \frac{18}{35} \hat{n} \cdot \vec{S}_1 \vec{S}_1 \cdot \vec{v}_1 + \frac{6}{5} \hat{n} \cdot \vec{S}_1 \vec{S}_1 \cdot \vec{v}_2}{r^4} \right) \frac{1}{\epsilon_d} \left\{ \right.$$

{DiagS1S1[3, 1, 8],

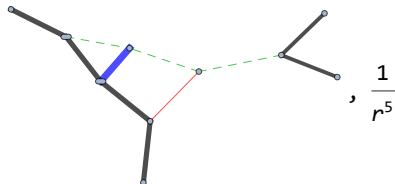

$$G^3 m_1 m_2 \left( - \frac{32}{7} \vec{v}_1 \cdot \vec{v}_2 \left( \hat{n} \cdot \vec{S}_1 \right)^2 + 12 \hat{n} \cdot \vec{S}_1 \hat{n} \cdot \vec{v}_2 \vec{S}_1 \cdot \vec{v}_1 + \frac{80}{7} \hat{n} \cdot \vec{S}_1 \hat{n} \cdot \vec{v}_1 \vec{S}_1 \cdot \vec{v}_2 - \right.$$

$$\frac{148}{7} \vec{S}_1 \cdot \vec{S}_1 \hat{n} \cdot \vec{v}_1 \hat{n} \cdot \vec{v}_2 - \frac{236}{35} \vec{S}_1 \cdot \vec{v}_1 \vec{S}_1 \cdot \vec{v}_2 + \frac{188}{35} \vec{S}_1 \cdot \vec{S}_1 \vec{v}_1 \cdot \vec{v}_2 \Big) \Big\}$$

{DiagS1S1[3, 1, 9],

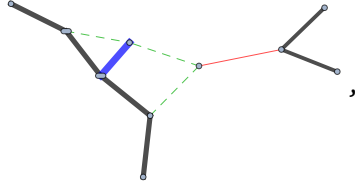

$$\frac{G^3 m_1 m_2 \left( \frac{8}{7} \vec{v}_1 \cdot \vec{v}_1 \left( \hat{n} \cdot \vec{S}_1 \right)^2 - \frac{44}{7} \hat{n} \cdot \vec{S}_1 \hat{n} \cdot \vec{v}_1 \vec{S}_1 \cdot \vec{v}_1 + 4 \vec{S}_1 \cdot \vec{S}_1 \left( \hat{n} \cdot \vec{v}_1 \right)^2 + \frac{64}{35} \left( \vec{S}_1 \cdot \vec{v}_1 \right)^2 - \frac{32}{35} \vec{S}_1 \cdot \vec{S}_1 \vec{v}_1 \cdot \vec{v}_1 \right)}{r^5} \Big\}$$

{DiagS1S1[3, 1, 10],

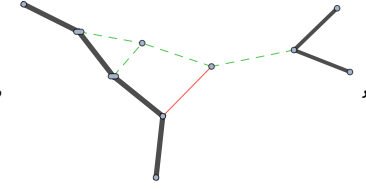

$$\begin{aligned} & G^3 m_1 m_2 \left( \frac{-8 \hat{n} \cdot \vec{S}_1 \hat{n} \cdot \vec{S}_1 \hat{n} \cdot \vec{v}_2 + \frac{68}{25} \vec{S}_1 \cdot \vec{S}_1 \hat{n} \cdot \vec{v}_2 + \frac{68}{25} \hat{n} \cdot \vec{S}_1 \vec{S}_1 \cdot \vec{v}_2 - \frac{16}{5} \hat{n} \cdot \vec{S}_1 \vec{S}_1 \cdot \vec{a}_2 + \frac{12}{5} \hat{n} \cdot \vec{a}_2 \vec{S}_1 \cdot \vec{S}_1 + \frac{68}{25} \hat{n} \cdot \vec{S}_1 \vec{S}_1 \cdot \vec{v}_2}{r^4} + \right. \\ & \frac{1}{r^5} \left( \frac{87}{4} \hat{n} \cdot \vec{v}_1 \hat{n} \cdot \vec{v}_2 \left( \hat{n} \cdot \vec{S}_1 \right)^2 - \frac{445}{196} \vec{v}_1 \cdot \vec{v}_2 \left( \hat{n} \cdot \vec{S}_1 \right)^2 - \frac{445}{98} \hat{n} \cdot \vec{v}_2 \vec{S}_1 \cdot \vec{v}_1 \hat{n} \cdot \vec{S}_1 - \frac{893}{98} \hat{n} \cdot \vec{v}_1 \vec{S}_1 \cdot \vec{v}_2 \hat{n} \cdot \vec{S}_1 - \right. \\ & 16 \hat{n} \cdot \vec{v}_2 \vec{S}_1 \cdot \vec{v}_2 \hat{n} \cdot \vec{S}_1 + \frac{16}{5} \left( \vec{S}_1 \cdot \vec{v}_2 \right)^2 - \frac{36}{7} \hat{n} \times \vec{S}_1 \cdot \vec{v}_1 \hat{n} \times \vec{S}_1 \cdot \vec{v}_2 + 12 \left( \hat{n} \cdot \vec{v}_2 \right)^2 \vec{S}_1 \cdot \vec{S}_1 - \\ & \frac{1033}{196} \hat{n} \cdot \vec{v}_1 \hat{n} \cdot \vec{v}_2 \vec{S}_1 \cdot \vec{S}_1 + \frac{3149 \vec{S}_1 \cdot \vec{v}_1 \vec{S}_1 \cdot \vec{v}_2}{2450} + \frac{3009 \vec{S}_1 \cdot \vec{S}_1 \vec{v}_1 \cdot \vec{v}_2}{4900} - \frac{12}{5} \vec{S}_1 \cdot \vec{S}_1 \vec{v}_2 \cdot \vec{v}_2 \Big) + \\ & \left( \frac{12 \hat{n} \cdot \vec{S}_1 \hat{n} \cdot \vec{S}_1 \hat{n} \cdot \vec{v}_2 - \frac{12}{5} \vec{S}_1 \cdot \vec{S}_1 \hat{n} \cdot \vec{v}_2 - \frac{12}{5} \hat{n} \cdot \vec{S}_1 \vec{S}_1 \cdot \vec{v}_2 - \frac{12}{5} \hat{n} \cdot \vec{S}_1 \vec{S}_1 \cdot \vec{v}_2}{r^4} + \frac{1}{r^5} \right. \\ & \left( -27 \hat{n} \cdot \vec{v}_1 \hat{n} \cdot \vec{v}_2 \left( \hat{n} \cdot \vec{S}_1 \right)^2 + \frac{27}{7} \vec{v}_1 \cdot \vec{v}_2 \left( \hat{n} \cdot \vec{S}_1 \right)^2 + \frac{54}{7} \hat{n} \cdot \vec{v}_2 \vec{S}_1 \cdot \vec{v}_1 \hat{n} \cdot \vec{S}_1 + \frac{54}{7} \hat{n} \cdot \vec{v}_1 \vec{S}_1 \cdot \vec{v}_2 \hat{n} \cdot \vec{S}_1 + \right. \\ & \left. \frac{27}{7} \hat{n} \cdot \vec{v}_1 \hat{n} \cdot \vec{v}_2 \vec{S}_1 \cdot \vec{S}_1 - \frac{54}{35} \vec{S}_1 \cdot \vec{v}_1 \vec{S}_1 \cdot \vec{v}_2 - \frac{27}{35} \vec{S}_1 \cdot \vec{S}_1 \vec{v}_1 \cdot \vec{v}_2 \right) \log \left( \frac{r}{R_\theta} \right) + \\ & \frac{1}{\epsilon_d} \left( \frac{-4 \hat{n} \cdot \vec{S}_1 \hat{n} \cdot \vec{S}_1 \hat{n} \cdot \vec{v}_2 + \frac{4}{5} \vec{S}_1 \cdot \vec{S}_1 \hat{n} \cdot \vec{v}_2 + \frac{4}{5} \hat{n} \cdot \vec{S}_1 \vec{S}_1 \cdot \vec{v}_2 + \frac{4}{5} \hat{n} \cdot \vec{S}_1 \vec{S}_1 \cdot \vec{v}_2}{r^4} + \frac{1}{r^5} \right. \\ & \left( 9 \hat{n} \cdot \vec{v}_1 \hat{n} \cdot \vec{v}_2 \left( \hat{n} \cdot \vec{S}_1 \right)^2 - \frac{9}{7} \vec{v}_1 \cdot \vec{v}_2 \left( \hat{n} \cdot \vec{S}_1 \right)^2 - \frac{18}{7} \hat{n} \cdot \vec{v}_2 \vec{S}_1 \cdot \vec{v}_1 \hat{n} \cdot \vec{S}_1 - \right. \\ & \left. \left. \frac{18}{7} \hat{n} \cdot \vec{v}_1 \vec{S}_1 \cdot \vec{v}_2 \hat{n} \cdot \vec{S}_1 - \frac{9}{7} \hat{n} \cdot \vec{v}_1 \hat{n} \cdot \vec{v}_2 \vec{S}_1 \cdot \vec{S}_1 + \frac{18}{35} \vec{S}_1 \cdot \vec{v}_1 \vec{S}_1 \cdot \vec{v}_2 + \frac{9}{35} \vec{S}_1 \cdot \vec{S}_1 \vec{v}_1 \cdot \vec{v}_2 \right) \right) \Big\} \end{aligned}$$

{DiagS1S1[3, 1, 11],

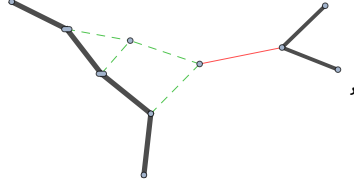

$$\begin{aligned}
 & G^3 m_1 m_2 \left( \frac{\frac{72}{49} \hat{n} \cdot \vec{S}_1 \hat{n} \cdot \vec{S}_1 \hat{n} \cdot \vec{v}_1 - \frac{276 \vec{S}_1 \cdot \vec{S}_1 \hat{n} \cdot \vec{v}_1}{1225} - \frac{1116 \hat{n} \cdot \vec{S}_1 \vec{S}_1 \cdot \vec{v}_1}{1225} + \frac{8}{5} \hat{n} \cdot \vec{S}_1 \vec{S}_1 \cdot \vec{a}_1 - \frac{4}{5} \hat{n} \cdot \vec{a}_1 \vec{S}_1 \cdot \vec{S}_1 - \frac{1116 \hat{n} \cdot \vec{S}_1 \vec{S}_1 \cdot \vec{v}_1}{1225}}{r^4} + \right. \\
 & \frac{1}{r^5} \left( \frac{12}{7} (\hat{n} \times \vec{S}_1 \cdot \vec{v}_1)^2 - \frac{37}{12} (\hat{n} \cdot \vec{S}_1)^2 (\hat{n} \cdot \vec{v}_1)^2 - \frac{23 (\vec{S}_1 \cdot \vec{v}_1)^2}{7350} + \frac{1147}{588} (\hat{n} \cdot \vec{v}_1)^2 \vec{S}_1 \cdot \vec{S}_1 - \right. \\
 & 4 \hat{n} \cdot \vec{v}_1 \hat{n} \cdot \vec{v}_2 \vec{S}_1 \cdot \vec{S}_1 + \frac{55}{147} \hat{n} \cdot \vec{S}_1 \hat{n} \cdot \vec{v}_1 \vec{S}_1 \cdot \vec{v}_1 + 8 \hat{n} \cdot \vec{S}_1 \hat{n} \cdot \vec{v}_2 \vec{S}_1 \cdot \vec{v}_1 - \\
 & \left. \frac{8}{5} \vec{S}_1 \cdot \vec{v}_1 \vec{S}_1 \cdot \vec{v}_2 + \frac{727}{588} (\hat{n} \cdot \vec{S}_1)^2 \vec{v}_1 \cdot \vec{v}_1 - \frac{11363 \vec{S}_1 \cdot \vec{S}_1 \vec{v}_1 \cdot \vec{v}_1}{14700} + \frac{4}{5} \vec{S}_1 \cdot \vec{S}_1 \vec{v}_1 \cdot \vec{v}_2 \right) + \\
 & \left( \frac{-\frac{12}{7} \hat{n} \cdot \vec{S}_1 \hat{n} \cdot \vec{S}_1 \hat{n} \cdot \vec{v}_1 + \frac{12}{35} \vec{S}_1 \cdot \vec{S}_1 \hat{n} \cdot \vec{v}_1 + \frac{12}{35} \hat{n} \cdot \vec{S}_1 \vec{S}_1 \cdot \vec{v}_1 + \frac{12}{35} \hat{n} \cdot \vec{S}_1 \vec{S}_1 \cdot \vec{v}_1}{r^4} + \frac{1}{r^5} \left( 3 (\hat{n} \cdot \vec{v}_1)^2 (\hat{n} \cdot \vec{S}_1)^2 - \frac{3}{7} \vec{v}_1 \cdot \vec{v}_1 \right. \right. \\
 & \left. \left. (\hat{n} \cdot \vec{S}_1)^2 - \frac{12}{7} \hat{n} \cdot \vec{v}_1 \vec{S}_1 \cdot \vec{v}_1 \hat{n} \cdot \vec{S}_1 + \frac{6}{35} (\vec{S}_1 \cdot \vec{v}_1)^2 - \frac{3}{7} (\hat{n} \cdot \vec{v}_1)^2 \vec{S}_1 \cdot \vec{S}_1 + \frac{3}{35} \vec{S}_1 \cdot \vec{S}_1 \vec{v}_1 \cdot \vec{v}_1 \right) \log\left(\frac{r}{R_0}\right) + \frac{1}{\epsilon_d} \right. \\
 & \left. \left( \frac{\frac{4}{7} \hat{n} \cdot \vec{S}_1 \hat{n} \cdot \vec{S}_1 \hat{n} \cdot \vec{v}_1 - \frac{4}{35} \vec{S}_1 \cdot \vec{S}_1 \hat{n} \cdot \vec{v}_1 - \frac{4}{35} \hat{n} \cdot \vec{S}_1 \vec{S}_1 \cdot \vec{v}_1 - \frac{4}{35} \hat{n} \cdot \vec{S}_1 \vec{S}_1 \cdot \vec{v}_1}{r^4} + \frac{1}{r^5} \left( -(\hat{n} \cdot \vec{v}_1)^2 (\hat{n} \cdot \vec{S}_1)^2 + \right. \right. \right. \\
 & \left. \left. \frac{1}{7} \vec{v}_1 \cdot \vec{v}_1 (\hat{n} \cdot \vec{S}_1)^2 + \frac{4}{7} \hat{n} \cdot \vec{v}_1 \vec{S}_1 \cdot \vec{v}_1 \hat{n} \cdot \vec{S}_1 - \frac{2}{35} (\vec{S}_1 \cdot \vec{v}_1)^2 + \frac{1}{7} (\hat{n} \cdot \vec{v}_1)^2 \vec{S}_1 \cdot \vec{S}_1 - \frac{1}{35} \vec{S}_1 \cdot \vec{S}_1 \vec{v}_1 \cdot \vec{v}_1 \right) \right) \right) \Bigg\}
 \end{aligned}$$

{DiagS1S1[3, 1, 12],

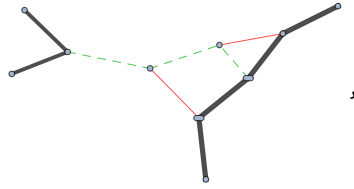

$$G^3 m_1 m_2 \left( -\frac{48}{7} \hat{n} \times \vec{S}_1 \cdot \vec{v}_1 \hat{n} \times \vec{S}_1 \cdot \vec{v}_2 + \frac{32}{7} \vec{S}_1 \cdot \vec{S}_1 \hat{n} \cdot \vec{v}_1 \hat{n} \cdot \vec{v}_2 - \frac{32}{7} \hat{n} \cdot \vec{S}_1 \hat{n} \cdot \vec{v}_2 \vec{S}_1 \cdot \vec{v}_1 + \frac{48}{35} \vec{S}_1 \cdot \vec{v}_1 \vec{S}_1 \cdot \vec{v}_2 - \frac{48}{35} \vec{S}_1 \cdot \vec{S}_1 \vec{v}_1 \cdot \vec{v}_2 \right) \Bigg\}$$

{DiagS1S1[3, 1, 13],

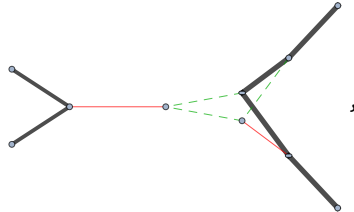

$$G^3 m_1 m_2 \left( -\frac{8}{7} \left( \hat{n} \times \vec{S}_1 \cdot \vec{v}_1 \right)^2 - \frac{40}{7} \vec{S}_1 \cdot \vec{S}_1 \left( \hat{n} \cdot \vec{v}_1 \right)^2 + \frac{40}{7} \hat{n} \cdot \vec{S}_1 \hat{n} \cdot \vec{v}_1 \vec{S}_1 \cdot \vec{v}_1 - \frac{192}{35} \left( \vec{S}_1 \cdot \vec{v}_1 \right)^2 + \frac{192}{35} \vec{S}_1 \cdot \vec{S}_1 \vec{v}_1 \cdot \vec{v}_1 \right) \frac{1}{r^5} \Bigg\}$$

{DiagS1S1[3, 1, 14], 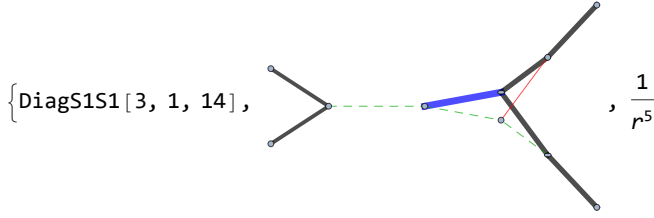 ,  $\frac{1}{r^5}$ }

$$G^3 m_1 m_2 \left( \frac{12}{7} \hat{n} \times \vec{S}_1 \cdot \vec{v}_1 \hat{n} \times \vec{S}_1 \cdot \vec{v}_2 + \frac{4}{7} \vec{v}_1 \cdot \vec{v}_2 \left( \hat{n} \cdot \vec{S}_1 \right)^2 + \frac{24}{7} \hat{n} \cdot \vec{S}_1 \hat{n} \cdot \vec{v}_2 \vec{S}_1 \cdot \vec{v}_1 + \frac{12}{7} \hat{n} \cdot \vec{S}_1 \hat{n} \cdot \vec{v}_1 \vec{S}_1 \cdot \vec{v}_2 - \frac{36}{7} \vec{S}_1 \cdot \vec{S}_1 \hat{n} \cdot \vec{v}_1 \hat{n} \cdot \vec{v}_2 - \frac{8}{7} \vec{S}_1 \cdot \vec{v}_1 \vec{S}_1 \cdot \vec{v}_2 - \frac{4}{35} \vec{S}_1 \cdot \vec{S}_1 \vec{v}_1 \cdot \vec{v}_2 \right) \frac{1}{r^5} \Bigg\}$$

{DiagS1S1[3, 1, 15], 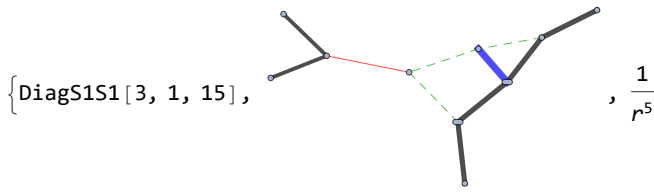 ,  $\frac{1}{r^5}$ }

$$G^3 m_1 m_2 \left( -\frac{2}{7} \left( \hat{n} \times \vec{S}_1 \cdot \vec{v}_1 \right)^2 + \frac{22}{7} \vec{S}_1 \cdot \vec{S}_1 \left( \hat{n} \cdot \vec{v}_1 \right)^2 - \frac{22}{7} \hat{n} \cdot \vec{S}_1 \hat{n} \cdot \vec{v}_1 \vec{S}_1 \cdot \vec{v}_1 + \frac{12}{7} \vec{v}_1 \cdot \vec{v}_1 \left( \hat{n} \cdot \vec{S}_1 \right)^2 + \frac{16}{7} \left( \vec{S}_1 \cdot \vec{v}_1 \right)^2 - \frac{44}{35} \vec{S}_1 \cdot \vec{S}_1 \vec{v}_1 \cdot \vec{v}_1 \right) \Bigg\}$$

{DiagS1S1[3, 1, 16], 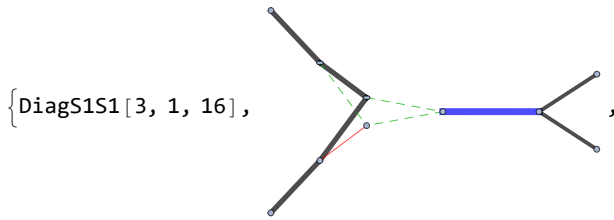 ,

$$G^3 m_1 m_2 \left( \frac{1}{r^5 \in_d} \left( -\frac{8}{3} \left( \hat{n} \cdot \vec{S}_1 \right)^2 \left( \hat{n} \cdot \vec{v}_2 \right)^2 + \frac{8}{21} \vec{v}_2 \cdot \vec{v}_2 \left( \hat{n} \cdot \vec{S}_1 \right)^2 + \frac{32}{21} \hat{n} \cdot \vec{S}_1 \hat{n} \cdot \vec{v}_2 \vec{S}_1 \cdot \vec{v}_2 + \frac{8}{21} \vec{S}_1 \cdot \vec{S}_1 \left( \hat{n} \cdot \vec{v}_2 \right)^2 - \frac{16}{105} \left( \vec{S}_1 \cdot \vec{v}_2 \right)^2 - \frac{8}{105} \vec{S}_1 \cdot \vec{S}_1 \vec{v}_2 \cdot \vec{v}_2 \right) + \frac{1}{r^5} \log \left( \frac{r}{R_\theta} \right) \left( 8 \left( \hat{n} \cdot \vec{S}_1 \right)^2 \left( \hat{n} \cdot \vec{v}_2 \right)^2 - \frac{8}{7} \vec{v}_2 \cdot \vec{v}_2 \left( \hat{n} \cdot \vec{S}_1 \right)^2 - \frac{32}{7} \hat{n} \cdot \vec{S}_1 \hat{n} \cdot \vec{v}_2 \vec{S}_1 \cdot \vec{v}_2 - \frac{8}{7} \vec{S}_1 \cdot \vec{S}_1 \left( \hat{n} \cdot \vec{v}_2 \right)^2 + \frac{16}{35} \left( \vec{S}_1 \cdot \vec{v}_2 \right)^2 + \frac{8}{35} \vec{S}_1 \cdot \vec{S}_1 \vec{v}_2 \cdot \vec{v}_2 \right) + \frac{1}{r^5} \left( -\frac{4}{7} \left( \hat{n} \times \vec{S}_1 \cdot \vec{v}_2 \right)^2 - 8 \left( \hat{n} \cdot \vec{S}_1 \right)^2 \left( \hat{n} \cdot \vec{v}_2 \right)^2 + \frac{20}{49} \vec{S}_1 \cdot \vec{S}_1 \left( \hat{n} \cdot \vec{v}_2 \right)^2 + \frac{940}{147} \hat{n} \cdot \vec{S}_1 \hat{n} \cdot \vec{v}_2 \vec{S}_1 \cdot \vec{v}_2 + \frac{4}{147} \vec{v}_2 \cdot \vec{v}_2 \left( \hat{n} \cdot \vec{S}_1 \right)^2 - \frac{1628}{1225} \left( \vec{S}_1 \cdot \vec{v}_2 \right)^2 + \frac{1688}{3675} \vec{S}_1 \cdot \vec{S}_1 \vec{v}_2 \cdot \vec{v}_2 \right) \right) \Bigg\}$$

{DiagS1S1[3, 1, 17], 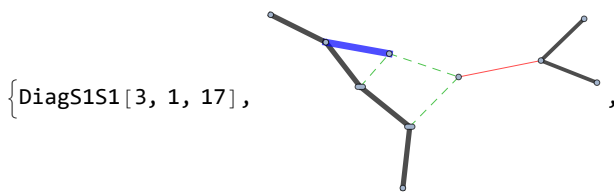 ,

$$G^3 m_1 m_2 \left( \frac{1}{r^5 \in_d} \left( -16 \left( \hat{n} \cdot \vec{S}_1 \right)^2 \left( \hat{n} \cdot \vec{v}_1 \right)^2 + \frac{16}{7} \vec{v}_1 \cdot \vec{v}_1 \left( \hat{n} \cdot \vec{S}_1 \right)^2 + \frac{64}{7} \hat{n} \cdot \vec{S}_1 \hat{n} \cdot \vec{v}_1 \vec{S}_1 \cdot \vec{v}_1 + \frac{16}{7} \vec{S}_1 \cdot \vec{S}_1 \left( \hat{n} \cdot \vec{v}_1 \right)^2 - \right. \right. \\ \left. \frac{32}{35} \left( \vec{S}_1 \cdot \vec{v}_1 \right)^2 - \frac{16}{35} \vec{S}_1 \cdot \vec{S}_1 \vec{v}_1 \cdot \vec{v}_1 \right) + \frac{1}{r^5} \log \left( \frac{r}{R_\theta} \right) \left( 48 \left( \hat{n} \cdot \vec{S}_1 \right)^2 \left( \hat{n} \cdot \vec{v}_1 \right)^2 - \frac{48}{7} \vec{v}_1 \cdot \vec{v}_1 \left( \hat{n} \cdot \vec{S}_1 \right)^2 - \right. \\ \left. \frac{192}{7} \hat{n} \cdot \vec{S}_1 \hat{n} \cdot \vec{v}_1 \vec{S}_1 \cdot \vec{v}_1 - \frac{48}{7} \vec{S}_1 \cdot \vec{S}_1 \left( \hat{n} \cdot \vec{v}_1 \right)^2 + \frac{96}{35} \left( \vec{S}_1 \cdot \vec{v}_1 \right)^2 + \frac{48}{35} \vec{S}_1 \cdot \vec{S}_1 \vec{v}_1 \cdot \vec{v}_1 \right) + \frac{1}{r^5} \\ \left( -\frac{22}{7} \left( \hat{n} \times \vec{S}_1 \cdot \vec{v}_1 \right)^2 - \frac{112}{3} \left( \hat{n} \cdot \vec{S}_1 \right)^2 \left( \hat{n} \cdot \vec{v}_1 \right)^2 - \frac{326}{147} \vec{S}_1 \cdot \vec{S}_1 \left( \hat{n} \cdot \vec{v}_1 \right)^2 + \frac{3190}{147} \hat{n} \cdot \vec{S}_1 \hat{n} \cdot \vec{v}_1 \vec{S}_1 \cdot \vec{v}_1 + \right. \\ \left. \frac{472}{147} \vec{v}_1 \cdot \vec{v}_1 \left( \hat{n} \cdot \vec{S}_1 \right)^2 - \frac{12784}{3675} \left( \vec{S}_1 \cdot \vec{v}_1 \right)^2 + \frac{12088}{3675} \vec{S}_1 \cdot \vec{S}_1 \vec{v}_1 \cdot \vec{v}_1 \right) \Bigg) \Bigg\}$$

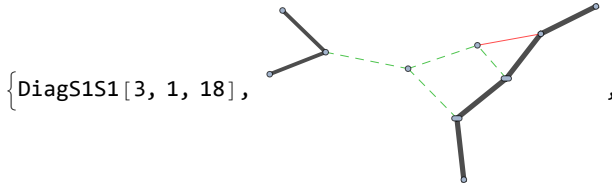

$$G^3 m_1 m_2 \left( \frac{-5 \hat{n} \cdot \vec{S}_1 \hat{n} \cdot \vec{S}_1 \hat{n} \cdot \vec{v}_2 + \frac{49}{25} \vec{S}_1 \cdot \vec{S}_1 \hat{n} \cdot \vec{v}_2 + \frac{29}{25} \hat{n} \cdot \vec{S}_1 \vec{S}_1 \cdot \vec{v}_2 - \frac{4}{5} \hat{n} \cdot \vec{S}_1 \vec{S}_1 \cdot \vec{a}_2 + \frac{4}{5} \hat{n} \cdot \vec{a}_2 \vec{S}_1 \cdot \vec{S}_1 + \frac{29}{25} \hat{n} \cdot \vec{S}_1 \vec{S}_1 \cdot \vec{v}_2}{r^4} + \right. \\ \frac{1}{r^5} \left( 16 \hat{n} \cdot \vec{v}_1 \hat{n} \cdot \vec{v}_2 \left( \hat{n} \cdot \vec{S}_1 \right)^2 - \frac{176}{147} \vec{v}_1 \cdot \vec{v}_2 \left( \hat{n} \cdot \vec{S}_1 \right)^2 - \frac{646}{147} \hat{n} \cdot \vec{v}_2 \vec{S}_1 \cdot \vec{v}_1 \hat{n} \cdot \vec{S}_1 - \frac{940}{147} \hat{n} \cdot \vec{v}_1 \vec{S}_1 \cdot \vec{v}_2 \hat{n} \cdot \vec{S}_1 - \right. \\ \left. 4 \hat{n} \cdot \vec{v}_2 \vec{S}_1 \cdot \vec{v}_2 \hat{n} \cdot \vec{S}_1 + \frac{4}{5} \left( \vec{S}_1 \cdot \vec{v}_2 \right)^2 - 2 \hat{n} \times \vec{S}_1 \cdot \vec{v}_1 \hat{n} \times \vec{S}_1 \cdot \vec{v}_2 + 4 \left( \hat{n} \cdot \vec{v}_2 \right)^2 \vec{S}_1 \cdot \vec{S}_1 - \right. \\ \left. \frac{138}{49} \hat{n} \cdot \vec{v}_1 \hat{n} \cdot \vec{v}_2 \vec{S}_1 \cdot \vec{S}_1 + \frac{1156}{1225} \vec{S}_1 \cdot \vec{v}_1 \vec{S}_1 \cdot \vec{v}_2 + \frac{404}{3675} \vec{S}_1 \cdot \vec{S}_1 \vec{v}_1 \cdot \vec{v}_2 - \frac{4}{5} \vec{S}_1 \cdot \vec{S}_1 \vec{v}_2 \cdot \vec{v}_2 \right) + \\ \left( \frac{6 \hat{n} \cdot \vec{S}_1 \hat{n} \cdot \vec{S}_1 \hat{n} \cdot \vec{v}_2 - \frac{6}{5} \vec{S}_1 \cdot \vec{S}_1 \hat{n} \cdot \vec{v}_2 - \frac{6}{5} \hat{n} \cdot \vec{S}_1 \vec{S}_1 \cdot \vec{v}_2 - \frac{6}{5} \hat{n} \cdot \vec{S}_1 \vec{S}_1 \cdot \vec{v}_2}{r^4} + \frac{1}{r^5} \right. \\ \left( -16 \hat{n} \cdot \vec{v}_1 \hat{n} \cdot \vec{v}_2 \left( \hat{n} \cdot \vec{S}_1 \right)^2 + \frac{16}{7} \vec{v}_1 \cdot \vec{v}_2 \left( \hat{n} \cdot \vec{S}_1 \right)^2 + \frac{32}{7} \hat{n} \cdot \vec{v}_2 \vec{S}_1 \cdot \vec{v}_1 \hat{n} \cdot \vec{S}_1 + \frac{32}{7} \hat{n} \cdot \vec{v}_1 \vec{S}_1 \cdot \vec{v}_2 \hat{n} \cdot \vec{S}_1 + \right. \\ \left. \frac{16}{7} \hat{n} \cdot \vec{v}_1 \hat{n} \cdot \vec{v}_2 \vec{S}_1 \cdot \vec{S}_1 - \frac{32}{35} \vec{S}_1 \cdot \vec{v}_1 \vec{S}_1 \cdot \vec{v}_2 - \frac{16}{35} \vec{S}_1 \cdot \vec{S}_1 \vec{v}_1 \cdot \vec{v}_2 \right) \log \left( \frac{r}{R_\theta} \right) + \\ \left. \frac{1}{r^5} \left( \frac{-2 \hat{n} \cdot \vec{S}_1 \hat{n} \cdot \vec{S}_1 \hat{n} \cdot \vec{v}_2 + \frac{2}{5} \vec{S}_1 \cdot \vec{S}_1 \hat{n} \cdot \vec{v}_2 + \frac{2}{5} \hat{n} \cdot \vec{S}_1 \vec{S}_1 \cdot \vec{v}_2 + \frac{2}{5} \hat{n} \cdot \vec{S}_1 \vec{S}_1 \cdot \vec{v}_2}{r^4} + \frac{1}{r^5} \right. \right. \\ \left. \left( \frac{16}{3} \hat{n} \cdot \vec{v}_1 \hat{n} \cdot \vec{v}_2 \left( \hat{n} \cdot \vec{S}_1 \right)^2 - \frac{16}{21} \vec{v}_1 \cdot \vec{v}_2 \left( \hat{n} \cdot \vec{S}_1 \right)^2 - \frac{32}{21} \hat{n} \cdot \vec{v}_2 \vec{S}_1 \cdot \vec{v}_1 \hat{n} \cdot \vec{S}_1 - \right. \right. \\ \left. \left. \frac{32}{21} \hat{n} \cdot \vec{v}_1 \vec{S}_1 \cdot \vec{v}_2 \hat{n} \cdot \vec{S}_1 - \frac{16}{21} \hat{n} \cdot \vec{v}_1 \hat{n} \cdot \vec{v}_2 \vec{S}_1 \cdot \vec{S}_1 + \frac{32}{105} \vec{S}_1 \cdot \vec{v}_1 \vec{S}_1 \cdot \vec{v}_2 + \frac{16}{105} \vec{S}_1 \cdot \vec{S}_1 \vec{v}_1 \cdot \vec{v}_2 \right) \right) \Bigg) \Bigg\}$$

{DiagS1S1[3, 1, 19],

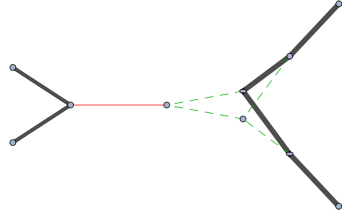

,  $G^3 m_1 m_2$

$$\left( \frac{-\frac{173}{49} \hat{n} \cdot \vec{S}_1 \hat{n} \cdot \vec{S}_1 \hat{n} \cdot \vec{v}_1 + \frac{327}{245} \vec{S}_1 \cdot \vec{S}_1 \hat{n} \cdot \vec{v}_1 + \frac{1041}{245} \hat{n} \cdot \vec{S}_1 \vec{S}_1 \cdot \vec{v}_1 + \frac{2}{5} \hat{n} \cdot \vec{S}_1 \vec{S}_1 \cdot \vec{a}_1 - \frac{2}{5} \hat{n} \cdot \vec{a}_1 \vec{S}_1 \cdot \vec{S}_1 - \frac{1017}{245} \hat{n} \cdot \vec{S}_1 \vec{S}_1 \cdot \vec{v}_1}{r^4} + \right.$$

$$\frac{1}{r^5} \left( \frac{64}{7} (\hat{n} \times \vec{S}_1 \cdot \vec{v}_1)^2 + \frac{23}{3} (\hat{n} \cdot \vec{S}_1)^2 (\hat{n} \cdot \vec{v}_1)^2 + \frac{15038 (\vec{S}_1 \cdot \vec{v}_1)^2}{3675} + 67 (\hat{n} \cdot \vec{S}_1)^2 \hat{n} \cdot \vec{v}_1 \hat{n} \cdot \vec{v}_2 + \frac{907}{147} (\hat{n} \cdot \vec{v}_1)^2 \vec{S}_1 \cdot \vec{S}_1 - \right.$$

$$\frac{281}{49} \hat{n} \cdot \vec{v}_1 \hat{n} \cdot \vec{v}_2 \vec{S}_1 \cdot \vec{S}_1 - \frac{1328}{147} \hat{n} \cdot \vec{S}_1 \hat{n} \cdot \vec{v}_1 \vec{S}_1 \cdot \vec{v}_1 - \frac{730}{49} \hat{n} \cdot \vec{S}_1 \hat{n} \cdot \vec{v}_2 \vec{S}_1 \cdot \vec{v}_1 - \frac{758}{49} \hat{n} \cdot \vec{S}_1 \hat{n} \cdot \vec{v}_1 \vec{S}_1 \cdot \vec{v}_2 +$$

$$\frac{478}{245} \vec{S}_1 \cdot \vec{v}_1 \vec{S}_1 \cdot \vec{v}_2 + \frac{25}{147} (\hat{n} \cdot \vec{S}_1)^2 \vec{v}_1 \cdot \vec{v}_1 - \frac{25661 \vec{S}_1 \cdot \vec{S}_1 \vec{v}_1 \cdot \vec{v}_1}{3675} - \frac{379}{49} (\hat{n} \cdot \vec{S}_1)^2 \vec{v}_1 \cdot \vec{v}_2 + \frac{31}{49} \vec{S}_1 \cdot \vec{S}_1 \vec{v}_1 \cdot \vec{v}_2 \Big) +$$

$$\left( \frac{\frac{30}{7} \hat{n} \cdot \vec{S}_1 \hat{n} \cdot \vec{S}_1 \hat{n} \cdot \vec{v}_1 - \frac{6}{7} \vec{S}_1 \cdot \vec{S}_1 \hat{n} \cdot \vec{v}_1 - \frac{6}{7} \hat{n} \cdot \vec{S}_1 \vec{S}_1 \cdot \vec{v}_1 - \frac{6}{7} \hat{n} \cdot \vec{S}_1 \vec{S}_1 \cdot \vec{v}_1}{r^4} + \frac{1}{r^5} \right.$$

$$\left( -6 (\hat{n} \cdot \vec{v}_1)^2 (\hat{n} \cdot \vec{S}_1)^2 - 90 \hat{n} \cdot \vec{v}_1 \hat{n} \cdot \vec{v}_2 (\hat{n} \cdot \vec{S}_1)^2 + \frac{6}{7} \vec{v}_1 \cdot \vec{v}_1 (\hat{n} \cdot \vec{S}_1)^2 + \frac{90}{7} \vec{v}_1 \cdot \vec{v}_2 (\hat{n} \cdot \vec{S}_1)^2 + \right.$$

$$\frac{24}{7} \hat{n} \cdot \vec{v}_1 \vec{S}_1 \cdot \vec{v}_1 \hat{n} \cdot \vec{S}_1 + \frac{180}{7} \hat{n} \cdot \vec{v}_2 \vec{S}_1 \cdot \vec{v}_1 \hat{n} \cdot \vec{S}_1 + \frac{180}{7} \hat{n} \cdot \vec{v}_1 \vec{S}_1 \cdot \vec{v}_2 \hat{n} \cdot \vec{S}_1 - \frac{12}{35} (\vec{S}_1 \cdot \vec{v}_1)^2 +$$

$$\frac{6}{7} (\hat{n} \cdot \vec{v}_1)^2 \vec{S}_1 \cdot \vec{S}_1 + \frac{90}{7} \hat{n} \cdot \vec{v}_1 \hat{n} \cdot \vec{v}_2 \vec{S}_1 \cdot \vec{S}_1 - \frac{36}{7} \vec{S}_1 \cdot \vec{v}_1 \vec{S}_1 \cdot \vec{v}_2 - \frac{6}{35} \vec{S}_1 \cdot \vec{S}_1 \vec{v}_1 \cdot \vec{v}_1 - \frac{18}{7} \vec{S}_1 \cdot \vec{S}_1 \vec{v}_1 \cdot \vec{v}_2 \Big) \Bigg)$$

$$\log\left(\frac{r}{R_\theta}\right) + \frac{1}{\epsilon_d} \left( \frac{-\frac{10}{7} \hat{n} \cdot \vec{S}_1 \hat{n} \cdot \vec{S}_1 \hat{n} \cdot \vec{v}_1 + \frac{2}{7} \vec{S}_1 \cdot \vec{S}_1 \hat{n} \cdot \vec{v}_1 + \frac{2}{7} \hat{n} \cdot \vec{S}_1 \vec{S}_1 \cdot \vec{v}_1 + \frac{2}{7} \hat{n} \cdot \vec{S}_1 \vec{S}_1 \cdot \vec{v}_1}{r^4} + \frac{1}{r^5} \right.$$

$$\left( 2 (\hat{n} \cdot \vec{v}_1)^2 (\hat{n} \cdot \vec{S}_1)^2 + 30 \hat{n} \cdot \vec{v}_1 \hat{n} \cdot \vec{v}_2 (\hat{n} \cdot \vec{S}_1)^2 - \frac{2}{7} \vec{v}_1 \cdot \vec{v}_1 (\hat{n} \cdot \vec{S}_1)^2 - \frac{30}{7} \vec{v}_1 \cdot \vec{v}_2 (\hat{n} \cdot \vec{S}_1)^2 - \right.$$

$$\frac{8}{7} \hat{n} \cdot \vec{v}_1 \vec{S}_1 \cdot \vec{v}_1 \hat{n} \cdot \vec{S}_1 - \frac{60}{7} \hat{n} \cdot \vec{v}_2 \vec{S}_1 \cdot \vec{v}_1 \hat{n} \cdot \vec{S}_1 - \frac{60}{7} \hat{n} \cdot \vec{v}_1 \vec{S}_1 \cdot \vec{v}_2 \hat{n} \cdot \vec{S}_1 + \frac{4}{35} (\vec{S}_1 \cdot \vec{v}_1)^2 -$$

$$\frac{2}{7} (\hat{n} \cdot \vec{v}_1)^2 \vec{S}_1 \cdot \vec{S}_1 - \frac{30}{7} \hat{n} \cdot \vec{v}_1 \hat{n} \cdot \vec{v}_2 \vec{S}_1 \cdot \vec{S}_1 + \frac{12}{7} \vec{S}_1 \cdot \vec{v}_1 \vec{S}_1 \cdot \vec{v}_2 + \frac{2}{35} \vec{S}_1 \cdot \vec{S}_1 \vec{v}_1 \cdot \vec{v}_1 + \frac{6}{7} \vec{S}_1 \cdot \vec{S}_1 \vec{v}_1 \cdot \vec{v}_2 \Big) \Bigg) \Bigg\}$$

{DiagS1S1[3, 1, 20],

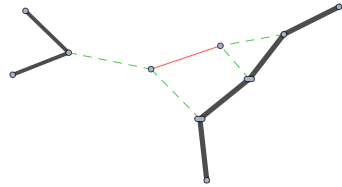

,

$$\frac{G^3 m_1 m_2 \left( -\frac{8}{7} \hat{n} \cdot \vec{S}_1 \cdot \vec{v}_1 \hat{n} \cdot \vec{S}_1 \cdot \vec{v}_2 + \frac{24}{7} \vec{S}_1 \cdot \vec{S}_1 \hat{n} \cdot \vec{v}_1 \hat{n} \cdot \vec{v}_2 - \frac{24}{7} \hat{n} \cdot \vec{S}_1 \hat{n} \cdot \vec{v}_2 \vec{S}_1 \cdot \vec{v}_1 + \frac{64}{35} \vec{S}_1 \cdot \vec{v}_1 \vec{S}_1 \cdot \vec{v}_2 - \frac{64}{35} \vec{S}_1 \cdot \vec{S}_1 \vec{v}_1 \cdot \vec{v}_2 \right)}{r^5} \Bigg\}$$

{DiagS1S1[3, 1, 21],

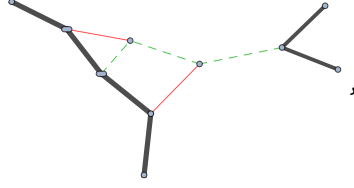

$$\frac{G^3 m_1 m_2 \left( 16 \vec{S}_1 \cdot \vec{S}_1 \hat{n} \cdot \vec{v}_1 \hat{n} \cdot \vec{v}_2 - 16 \hat{n} \cdot \vec{S}_1 \hat{n} \cdot \vec{v}_2 \vec{S}_1 \cdot \vec{v}_1 - \frac{48}{5} \vec{S}_1 \cdot \vec{S}_1 \vec{v}_1 \cdot \vec{v}_2 + \frac{48}{5} \vec{S}_1 \cdot \vec{v}_1 \vec{S}_1 \cdot \vec{v}_2 \right)}{r^5}$$

{DiagS1S1[3, 1, 22],

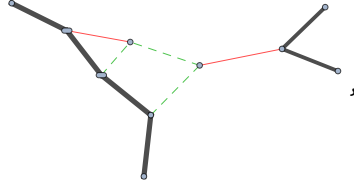

$$\frac{G^3 m_1 m_2 \left( -\frac{16}{7} \vec{S}_1 \cdot \vec{S}_1 (\hat{n} \cdot \vec{v}_1)^2 + \frac{16}{7} \hat{n} \cdot \vec{S}_1 \hat{n} \cdot \vec{v}_1 \vec{S}_1 \cdot \vec{v}_1 - \frac{64}{35} (\vec{S}_1 \cdot \vec{v}_1)^2 + \frac{64}{35} \vec{S}_1 \cdot \vec{S}_1 \vec{v}_1 \cdot \vec{v}_1 \right)}{r^5}$$

{DiagS1S1[3, 1, 23],

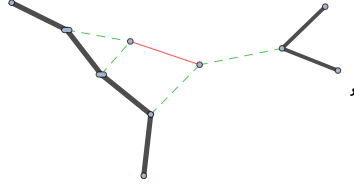

$$\frac{G^3 m_1 m_2 \left( -\frac{32}{7} \vec{v}_1 \cdot \vec{v}_2 (\hat{n} \cdot \vec{S}_1)^2 - \frac{16}{7} \hat{n} \cdot \vec{S}_1 \hat{n} \cdot \vec{v}_2 \vec{S}_1 \cdot \vec{v}_1 + \frac{16}{7} \hat{n} \cdot \vec{S}_1 \hat{n} \cdot \vec{v}_1 \vec{S}_1 \cdot \vec{v}_2 + \frac{16}{35} \vec{S}_1 \cdot \vec{S}_1 \vec{v}_1 \cdot \vec{v}_2 \right)}{r^5}$$

{DiagS1S1[3, 1, 24],

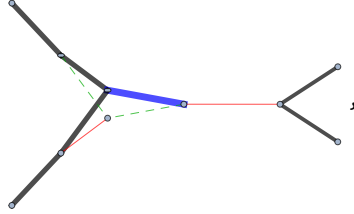

$$G^3 m_1 m_2 \left( \frac{-5 \hat{n} \cdot \vec{S}_1 \hat{n} \cdot \vec{S}_1 \hat{n} \cdot \vec{v}_1 + \frac{79}{25} \vec{S}_1 \cdot \vec{S}_1 \hat{n} \cdot \vec{v}_1 + \frac{19}{25} \hat{n} \cdot \vec{S}_1 \vec{S}_1 \cdot \vec{v}_1 + \frac{9}{25} \hat{n} \cdot \vec{S}_1 \vec{S}_1 \cdot \vec{v}_1}{r^4} + \frac{1}{r^5} \right. \\ \left( \frac{8}{7} (\hat{n} \cdot \vec{S}_1 \cdot \vec{v}_1)^2 + 24 (\hat{n} \cdot \vec{S}_1)^2 (\hat{n} \cdot \vec{v}_1)^2 + \frac{1034 (\vec{S}_1 \cdot \vec{v}_1)^2}{1225} - 24 (\hat{n} \cdot \vec{S}_1)^2 \hat{n} \cdot \vec{v}_1 \hat{n} \cdot \vec{v}_2 - \frac{494}{49} (\hat{n} \cdot \vec{v}_1)^2 \vec{S}_1 \cdot \vec{S}_1 + \right. \\ \frac{536}{49} \hat{n} \cdot \vec{v}_1 \hat{n} \cdot \vec{v}_2 \vec{S}_1 \cdot \vec{S}_1 - \frac{506}{49} \hat{n} \cdot \vec{S}_1 \hat{n} \cdot \vec{v}_1 \vec{S}_1 \cdot \vec{v}_1 + \frac{176}{49} \hat{n} \cdot \vec{S}_1 \hat{n} \cdot \vec{v}_2 \vec{S}_1 \cdot \vec{v}_1 + \frac{288}{49} \hat{n} \cdot \vec{S}_1 \hat{n} \cdot \vec{v}_1 \vec{S}_1 \cdot \vec{v}_2 - \\ \left. \frac{544 \vec{S}_1 \cdot \vec{v}_1 \vec{S}_1 \cdot \vec{v}_2}{1225} - \frac{144}{49} (\hat{n} \cdot \vec{S}_1)^2 \vec{v}_1 \cdot \vec{v}_1 + \frac{2022 \vec{S}_1 \cdot \vec{S}_1 \vec{v}_1 \cdot \vec{v}_1}{1225} + \frac{144}{49} (\hat{n} \cdot \vec{S}_1)^2 \vec{v}_1 \cdot \vec{v}_2 - \frac{2512 \vec{S}_1 \cdot \vec{S}_1 \vec{v}_1 \cdot \vec{v}_2}{1225} \right) + \\ \left( \frac{6 \hat{n} \cdot \vec{S}_1 \hat{n} \cdot \vec{S}_1 \hat{n} \cdot \vec{v}_1 - \frac{6}{5} \vec{S}_1 \cdot \vec{S}_1 \hat{n} \cdot \vec{v}_1 - \frac{6}{5} \hat{n} \cdot \vec{S}_1 \vec{S}_1 \cdot \vec{v}_1 - \frac{6}{5} \hat{n} \cdot \vec{S}_1 \vec{S}_1 \cdot \vec{v}_1}{r^4} + \frac{1}{r^5} \right. \\ \left. \left( -24 (\hat{n} \cdot \vec{v}_1)^2 (\hat{n} \cdot \vec{S}_1)^2 + 24 \hat{n} \cdot \vec{v}_1 \hat{n} \cdot \vec{v}_2 (\hat{n} \cdot \vec{S}_1)^2 + \frac{24}{7} \vec{v}_1 \cdot \vec{v}_1 (\hat{n} \cdot \vec{S}_1)^2 - \frac{24}{7} \vec{v}_1 \cdot \vec{v}_2 (\hat{n} \cdot \vec{S}_1)^2 + \right. \right.$$

$$\begin{aligned}
& \frac{96}{7} \hat{n} \cdot \vec{v}_1 \vec{S}_1 \cdot \vec{v}_1 \hat{n} \cdot \vec{S}_1 - \frac{48}{7} \hat{n} \cdot \vec{v}_2 \vec{S}_1 \cdot \vec{v}_1 \hat{n} \cdot \vec{S}_1 - \frac{48}{7} \hat{n} \cdot \vec{v}_1 \vec{S}_1 \cdot \vec{v}_2 \hat{n} \cdot \vec{S}_1 - \frac{48}{35} (\vec{S}_1 \cdot \vec{v}_1)^2 + \frac{24}{7} (\hat{n} \cdot \vec{v}_1)^2 \vec{S}_1 \cdot \vec{S}_1 - \\
& \left. \frac{24}{7} \hat{n} \cdot \vec{v}_1 \hat{n} \cdot \vec{v}_2 \vec{S}_1 \cdot \vec{S}_1 + \frac{48}{35} \vec{S}_1 \cdot \vec{v}_1 \vec{S}_1 \cdot \vec{v}_2 - \frac{24}{35} \vec{S}_1 \cdot \vec{S}_1 \vec{v}_1 \cdot \vec{v}_1 + \frac{24}{35} \vec{S}_1 \cdot \vec{S}_1 \vec{v}_1 \cdot \vec{v}_2 \right) \log \left( \frac{r}{R_\theta} \right) + \\
& \frac{1}{\epsilon_d} \left( \frac{-2 \hat{n} \cdot \vec{S}_1 \hat{n} \cdot \vec{S}_1 \hat{n} \cdot \vec{v}_1 + \frac{2}{5} \vec{S}_1 \cdot \vec{S}_1 \hat{n} \cdot \vec{v}_1 + \frac{2}{5} \hat{n} \cdot \vec{S}_1 \vec{S}_1 \cdot \vec{v}_1 + \frac{2}{5} \hat{n} \cdot \vec{S}_1 \vec{S}_1 \cdot \vec{v}_1}{r^4} + \frac{1}{r^5} \right. \\
& \left( 8 (\hat{n} \cdot \vec{v}_1)^2 (\hat{n} \cdot \vec{S}_1)^2 - 8 \hat{n} \cdot \vec{v}_1 \hat{n} \cdot \vec{v}_2 (\hat{n} \cdot \vec{S}_1)^2 - \frac{8}{7} \vec{v}_1 \cdot \vec{v}_1 (\hat{n} \cdot \vec{S}_1)^2 + \frac{8}{7} \vec{v}_1 \cdot \vec{v}_2 (\hat{n} \cdot \vec{S}_1)^2 - \right. \\
& \left. \frac{32}{7} \hat{n} \cdot \vec{v}_1 \vec{S}_1 \cdot \vec{v}_1 \hat{n} \cdot \vec{S}_1 + \frac{16}{7} \hat{n} \cdot \vec{v}_2 \vec{S}_1 \cdot \vec{v}_1 \hat{n} \cdot \vec{S}_1 + \frac{16}{7} \hat{n} \cdot \vec{v}_1 \vec{S}_1 \cdot \vec{v}_2 \hat{n} \cdot \vec{S}_1 + \frac{16}{35} (\vec{S}_1 \cdot \vec{v}_1)^2 - \right. \\
& \left. \left. \frac{8}{7} (\hat{n} \cdot \vec{v}_1)^2 \vec{S}_1 \cdot \vec{S}_1 + \frac{8}{7} \hat{n} \cdot \vec{v}_1 \hat{n} \cdot \vec{v}_2 \vec{S}_1 \cdot \vec{S}_1 - \frac{16}{35} \vec{S}_1 \cdot \vec{v}_1 \vec{S}_1 \cdot \vec{v}_2 + \frac{8}{35} \vec{S}_1 \cdot \vec{S}_1 \vec{v}_1 \cdot \vec{v}_1 - \frac{8}{35} \vec{S}_1 \cdot \vec{S}_1 \vec{v}_1 \cdot \vec{v}_2 \right) \right) \Bigg\}
\end{aligned}$$

{DiagS1S1[3, 1, 25],

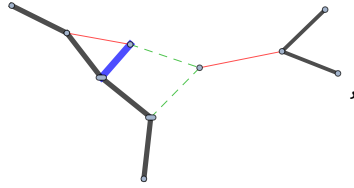

$$\begin{aligned}
& G^3 m_1 m_2 \left( \frac{-\frac{173}{49} \hat{n} \cdot \vec{S}_1 \hat{n} \cdot \vec{S}_1 \hat{n} \cdot \vec{v}_1 + \frac{229}{245} \vec{S}_1 \cdot \vec{S}_1 \hat{n} \cdot \vec{v}_1 - \frac{27}{49} \hat{n} \cdot \vec{S}_1 \vec{S}_1 \cdot \vec{v}_1 + \frac{257}{245} \hat{n} \cdot \vec{S}_1 \vec{S}_1 \cdot \vec{v}_1}{r^4} + \frac{1}{r^5} \right. \\
& \left( \frac{2}{7} (\hat{n} \cdot \vec{S}_1 \cdot \vec{v}_1)^2 + 29 (\hat{n} \cdot \vec{S}_1)^2 (\hat{n} \cdot \vec{v}_1)^2 + \frac{2}{49} (\vec{S}_1 \cdot \vec{v}_1)^2 - 29 (\hat{n} \cdot \vec{S}_1)^2 \hat{n} \cdot \vec{v}_1 \hat{n} \cdot \vec{v}_2 - \frac{313}{49} (\hat{n} \cdot \vec{v}_1)^2 \vec{S}_1 \cdot \vec{S}_1 + \right. \\
& \frac{271}{49} \hat{n} \cdot \vec{v}_1 \hat{n} \cdot \vec{v}_2 \vec{S}_1 \cdot \vec{S}_1 - \frac{510}{49} \hat{n} \cdot \vec{S}_1 \hat{n} \cdot \vec{v}_1 \vec{S}_1 \cdot \vec{v}_1 + \frac{206}{49} \hat{n} \cdot \vec{S}_1 \hat{n} \cdot \vec{v}_2 \vec{S}_1 \cdot \vec{v}_1 + \frac{346}{49} \hat{n} \cdot \vec{S}_1 \hat{n} \cdot \vec{v}_1 \vec{S}_1 \cdot \vec{v}_2 - \\
& \frac{122}{245} \vec{S}_1 \cdot \vec{v}_1 \vec{S}_1 \cdot \vec{v}_2 - \frac{173}{49} (\hat{n} \cdot \vec{S}_1)^2 \vec{v}_1 \cdot \vec{v}_1 + \frac{341}{245} \vec{S}_1 \cdot \vec{S}_1 \vec{v}_1 \cdot \vec{v}_1 + \frac{173}{49} (\hat{n} \cdot \vec{S}_1)^2 \vec{v}_1 \cdot \vec{v}_2 - \frac{229}{245} \vec{S}_1 \cdot \vec{S}_1 \vec{v}_1 \cdot \vec{v}_2 \Bigg) + \\
& \left( \frac{\frac{30}{7} \hat{n} \cdot \vec{S}_1 \hat{n} \cdot \vec{S}_1 \hat{n} \cdot \vec{v}_1 - \frac{6}{7} \vec{S}_1 \cdot \vec{S}_1 \hat{n} \cdot \vec{v}_1 - \frac{6}{7} \hat{n} \cdot \vec{S}_1 \vec{S}_1 \cdot \vec{v}_1 - \frac{6}{7} \hat{n} \cdot \vec{S}_1 \vec{S}_1 \cdot \vec{v}_1}{r^4} + \frac{1}{r^5} \right. \\
& \left( -30 (\hat{n} \cdot \vec{v}_1)^2 (\hat{n} \cdot \vec{S}_1)^2 + 30 \hat{n} \cdot \vec{v}_1 \hat{n} \cdot \vec{v}_2 (\hat{n} \cdot \vec{S}_1)^2 + \frac{30}{7} \vec{v}_1 \cdot \vec{v}_1 (\hat{n} \cdot \vec{S}_1)^2 - \frac{30}{7} \vec{v}_1 \cdot \vec{v}_2 (\hat{n} \cdot \vec{S}_1)^2 + \right. \\
& \frac{120}{7} \hat{n} \cdot \vec{v}_1 \vec{S}_1 \cdot \vec{v}_1 \hat{n} \cdot \vec{S}_1 - \frac{60}{7} \hat{n} \cdot \vec{v}_2 \vec{S}_1 \cdot \vec{v}_1 \hat{n} \cdot \vec{S}_1 - \frac{60}{7} \hat{n} \cdot \vec{v}_1 \vec{S}_1 \cdot \vec{v}_2 \hat{n} \cdot \vec{S}_1 - \frac{12}{7} (\vec{S}_1 \cdot \vec{v}_1)^2 + \\
& \left. \frac{30}{7} (\hat{n} \cdot \vec{v}_1)^2 \vec{S}_1 \cdot \vec{S}_1 - \frac{30}{7} \hat{n} \cdot \vec{v}_1 \hat{n} \cdot \vec{v}_2 \vec{S}_1 \cdot \vec{S}_1 + \frac{12}{7} \vec{S}_1 \cdot \vec{v}_1 \vec{S}_1 \cdot \vec{v}_2 - \frac{6}{7} \vec{S}_1 \cdot \vec{S}_1 \vec{v}_1 \cdot \vec{v}_1 + \frac{6}{7} \vec{S}_1 \cdot \vec{S}_1 \vec{v}_1 \cdot \vec{v}_2 \right) \Bigg) \\
& \log \left( \frac{r}{R_\theta} \right) + \frac{1}{\epsilon_d} \left( \frac{-\frac{10}{7} \hat{n} \cdot \vec{S}_1 \hat{n} \cdot \vec{S}_1 \hat{n} \cdot \vec{v}_1 + \frac{2}{7} \vec{S}_1 \cdot \vec{S}_1 \hat{n} \cdot \vec{v}_1 + \frac{2}{7} \hat{n} \cdot \vec{S}_1 \vec{S}_1 \cdot \vec{v}_1 + \frac{2}{7} \hat{n} \cdot \vec{S}_1 \vec{S}_1 \cdot \vec{v}_1}{r^4} + \frac{1}{r^5} \right. \\
& \left( 10 (\hat{n} \cdot \vec{v}_1)^2 (\hat{n} \cdot \vec{S}_1)^2 - 10 \hat{n} \cdot \vec{v}_1 \hat{n} \cdot \vec{v}_2 (\hat{n} \cdot \vec{S}_1)^2 - \frac{10}{7} \vec{v}_1 \cdot \vec{v}_1 (\hat{n} \cdot \vec{S}_1)^2 + \frac{10}{7} \vec{v}_1 \cdot \vec{v}_2 (\hat{n} \cdot \vec{S}_1)^2 - \right. \\
& \left. \frac{40}{7} \hat{n} \cdot \vec{v}_1 \vec{S}_1 \cdot \vec{v}_1 \hat{n} \cdot \vec{S}_1 + \frac{20}{7} \hat{n} \cdot \vec{v}_2 \vec{S}_1 \cdot \vec{v}_1 \hat{n} \cdot \vec{S}_1 + \frac{20}{7} \hat{n} \cdot \vec{v}_1 \vec{S}_1 \cdot \vec{v}_2 \hat{n} \cdot \vec{S}_1 + \frac{4}{7} (\vec{S}_1 \cdot \vec{v}_1)^2 - \right.
\end{aligned}$$

$$\left. \left. \left. \frac{10}{7} (\hat{n} \cdot \vec{v}_1)^2 \vec{S}_1 \cdot \vec{S}_1 + \frac{10}{7} \hat{n} \cdot \vec{v}_1 \hat{n} \cdot \vec{v}_2 \vec{S}_1 \cdot \vec{S}_1 - \frac{4}{7} \vec{S}_1 \cdot \vec{v}_1 \vec{S}_1 \cdot \vec{v}_2 + \frac{2}{7} \vec{S}_1 \cdot \vec{S}_1 \vec{v}_1 \cdot \vec{v}_1 - \frac{2}{7} \vec{S}_1 \cdot \vec{S}_1 \vec{v}_1 \cdot \vec{v}_2 \right) \right) \right\}$$

{DiagS1S1[3, 1, 26],

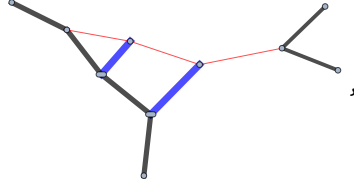

$$\frac{G^3 m_1 m_2 \left( \frac{2}{7} (\hat{n} \times \vec{S}_1 \cdot \vec{v}_1)^2 - \frac{11}{14} \vec{S}_1 \cdot \vec{S}_1 (\hat{n} \cdot \vec{v}_1)^2 + \frac{11}{14} \hat{n} \cdot \vec{S}_1 \hat{n} \cdot \vec{v}_1 \vec{S}_1 \cdot \vec{v}_1 - \frac{1}{10} (\vec{S}_1 \cdot \vec{v}_1)^2 + \frac{1}{10} \vec{S}_1 \cdot \vec{S}_1 \vec{v}_1 \cdot \vec{v}_1 \right)}{r^5}$$

{DiagS1S1[3, 1, 27],

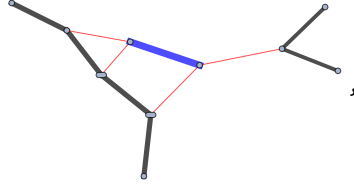

$$\frac{G^3 m_1 m_2 \left( \frac{12}{7} (\hat{n} \times \vec{S}_1 \cdot \vec{v}_1)^2 - \frac{36}{35} (\vec{S}_1 \cdot \vec{v}_1)^2 + \frac{36}{35} \vec{S}_1 \cdot \vec{S}_1 \vec{v}_1 \cdot \vec{v}_1 \right)}{r^5}$$

{DiagS1S1[3, 1, 28],

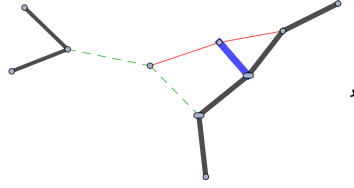

$$\frac{G^3 m_1 m_2 \left( \frac{2}{7} \hat{n} \times \vec{S}_1 \cdot \vec{v}_1 \hat{n} \times \vec{S}_1 \cdot \vec{v}_2 - \frac{6}{7} \vec{S}_1 \cdot \vec{S}_1 \hat{n} \cdot \vec{v}_1 \hat{n} \cdot \vec{v}_2 + \frac{6}{7} \hat{n} \cdot \vec{S}_1 \hat{n} \cdot \vec{v}_2 \vec{S}_1 \cdot \vec{v}_1 - \frac{16}{35} \vec{S}_1 \cdot \vec{v}_1 \vec{S}_1 \cdot \vec{v}_2 + \frac{16}{35} \vec{S}_1 \cdot \vec{S}_1 \vec{v}_1 \cdot \vec{v}_2 \right)}{r^5}$$

{DiagS1S1[3, 1, 29],

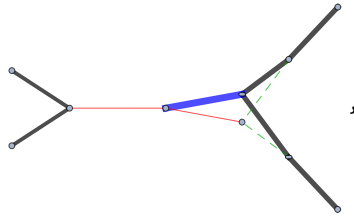

$$\frac{G^3 m_1 m_2 \left( -\frac{8}{7} (\hat{n} \times \vec{S}_1 \cdot \vec{v}_1)^2 + \frac{22}{7} \vec{S}_1 \cdot \vec{S}_1 (\hat{n} \cdot \vec{v}_1)^2 - \frac{22}{7} \hat{n} \cdot \vec{S}_1 \hat{n} \cdot \vec{v}_1 \vec{S}_1 \cdot \vec{v}_1 + \frac{2}{5} (\vec{S}_1 \cdot \vec{v}_1)^2 - \frac{2}{5} \vec{S}_1 \cdot \vec{S}_1 \vec{v}_1 \cdot \vec{v}_1 \right)}{r^5}$$

{DiagS1S1[3, 1, 30],

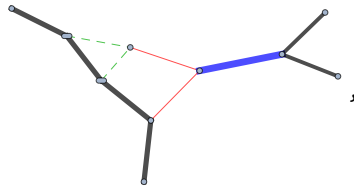

$$G^3 m_1 m_2 \left( \frac{1}{r^5 \in_d} \left( -\frac{4}{3} (\hat{n} \cdot \vec{S}_1)^2 (\hat{n} \cdot \vec{v}_2)^2 + \frac{4}{21} \vec{v}_2 \cdot \vec{v}_2 (\hat{n} \cdot \vec{S}_1)^2 + \frac{16}{21} \hat{n} \cdot \vec{S}_1 \hat{n} \cdot \vec{v}_2 \vec{S}_1 \cdot \vec{v}_2 + \frac{4}{21} \vec{S}_1 \cdot \vec{S}_1 (\hat{n} \cdot \vec{v}_2)^2 - \right. \right.$$

$$\frac{8}{105} \left( \vec{S}_1 \cdot \vec{v}_2 \right)^2 - \frac{4}{105} \vec{S}_1 \cdot \vec{S}_1 \vec{v}_2 \cdot \vec{v}_2 \Big) + \frac{1}{r^5} \log \left( \frac{r}{R_\theta} \right) \left( 4 \left( \hat{n} \cdot \vec{S}_1 \right)^2 \left( \hat{n} \cdot \vec{v}_2 \right)^2 - \frac{4}{7} \vec{v}_2 \cdot \vec{v}_2 \left( \hat{n} \cdot \vec{S}_1 \right)^2 - \right.$$

$$\left. \frac{16}{7} \hat{n} \cdot \vec{S}_1 \hat{n} \cdot \vec{v}_2 \vec{S}_1 \cdot \vec{v}_2 - \frac{4}{7} \vec{S}_1 \cdot \vec{S}_1 \left( \hat{n} \cdot \vec{v}_2 \right)^2 + \frac{8}{35} \left( \vec{S}_1 \cdot \vec{v}_2 \right)^2 + \frac{4}{35} \vec{S}_1 \cdot \vec{S}_1 \vec{v}_2 \cdot \vec{v}_2 \right) + \frac{-\frac{4}{3} \left( \hat{n} \cdot \vec{S}_1 \right)^2 \left( \hat{n} \cdot \vec{v}_2 \right)^2 - \frac{4}{49} \vec{v}_2 \cdot \vec{v}_2}{r^5}$$

{DiagS1S1[3, 1, 31],

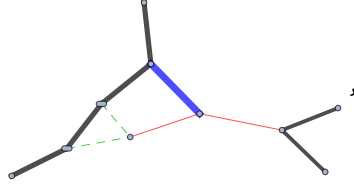

$$G^3 m_1 m_2 \left\{ \frac{1}{r^5 \in_d} \left( 12 \left( \hat{n} \cdot \vec{S}_1 \right)^2 \left( \hat{n} \cdot \vec{v}_1 \right)^2 - \frac{12}{7} \vec{v}_1 \cdot \vec{v}_1 \left( \hat{n} \cdot \vec{S}_1 \right)^2 - \frac{48}{7} \hat{n} \cdot \vec{S}_1 \hat{n} \cdot \vec{v}_1 \vec{S}_1 \cdot \vec{v}_1 - \frac{12}{7} \vec{S}_1 \cdot \vec{S}_1 \left( \hat{n} \cdot \vec{v}_1 \right)^2 + \right. \right.$$

$$\frac{24}{35} \left( \vec{S}_1 \cdot \vec{v}_1 \right)^2 + \frac{12}{35} \vec{S}_1 \cdot \vec{S}_1 \vec{v}_1 \cdot \vec{v}_1 \Big) + \frac{1}{r^5} \log \left( \frac{r}{R_\theta} \right) \left( -36 \left( \hat{n} \cdot \vec{S}_1 \right)^2 \left( \hat{n} \cdot \vec{v}_1 \right)^2 + \frac{36}{7} \vec{v}_1 \cdot \vec{v}_1 \left( \hat{n} \cdot \vec{S}_1 \right)^2 + \right.$$

$$\frac{144}{7} \hat{n} \cdot \vec{S}_1 \hat{n} \cdot \vec{v}_1 \vec{S}_1 \cdot \vec{v}_1 + \frac{36}{7} \vec{S}_1 \cdot \vec{S}_1 \left( \hat{n} \cdot \vec{v}_1 \right)^2 - \frac{72}{35} \left( \vec{S}_1 \cdot \vec{v}_1 \right)^2 - \frac{36}{35} \vec{S}_1 \cdot \vec{S}_1 \vec{v}_1 \cdot \vec{v}_1 \Big) +$$

$$\left. \frac{4 \left( \hat{n} \cdot \vec{S}_1 \right)^2 \left( \hat{n} \cdot \vec{v}_1 \right)^2 + \frac{8}{49} \vec{v}_1 \cdot \vec{v}_1 \left( \hat{n} \cdot \vec{S}_1 \right)^2 + \frac{4}{49} \hat{n} \cdot \vec{S}_1 \hat{n} \cdot \vec{v}_1 \vec{S}_1 \cdot \vec{v}_1 + \frac{8}{49} \vec{S}_1 \cdot \vec{S}_1 \left( \hat{n} \cdot \vec{v}_1 \right)^2 - \frac{444 \left( \vec{S}_1 \cdot \vec{v}_1 \right)^2}{1225} - \frac{292 \vec{S}_1 \cdot \vec{S}_1 \vec{v}_1 \cdot \vec{v}_1}{1225}}{r^5} \right\}$$

{DiagS1S1[3, 1, 32],

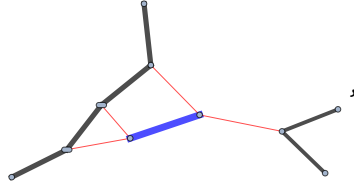

$$\frac{G^3 m_1 m_2 \left( \frac{10}{7} \left( \hat{n} \cdot \vec{S}_1 \cdot \vec{v}_1 \right)^2 + \frac{26}{35} \left( \vec{S}_1 \cdot \vec{v}_1 \right)^2 - \frac{26}{35} \vec{S}_1 \cdot \vec{S}_1 \vec{v}_1 \cdot \vec{v}_1 \right)}{r^5} \Big\}$$

{DiagS1S1[3, 1, 33],

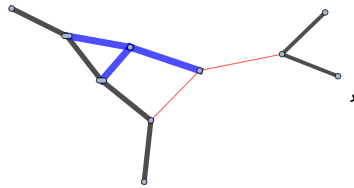

$$G^3 m_1 m_2 \left\{ \frac{1}{r^5 \in_d} \left( -3 \left( \hat{n} \cdot \vec{S}_1 \right)^2 \left( \hat{n} \cdot \vec{v}_1 \right)^2 + \frac{3}{7} \vec{v}_1 \cdot \vec{v}_1 \left( \hat{n} \cdot \vec{S}_1 \right)^2 + \frac{12}{7} \hat{n} \cdot \vec{S}_1 \hat{n} \cdot \vec{v}_1 \vec{S}_1 \cdot \vec{v}_1 + \right. \right.$$

$$\frac{3}{7} \vec{S}_1 \cdot \vec{S}_1 \left( \hat{n} \cdot \vec{v}_1 \right)^2 - \frac{6}{35} \left( \vec{S}_1 \cdot \vec{v}_1 \right)^2 - \frac{3}{35} \vec{S}_1 \cdot \vec{S}_1 \vec{v}_1 \cdot \vec{v}_1 \Big) + \frac{1}{r^5} \log \left( \frac{r}{R_\theta} \right) \left( 9 \left( \hat{n} \cdot \vec{S}_1 \right)^2 \left( \hat{n} \cdot \vec{v}_1 \right)^2 - \right.$$

$$\frac{9}{7} \vec{v}_1 \cdot \vec{v}_1 \left( \hat{n} \cdot \vec{S}_1 \right)^2 - \frac{36}{7} \hat{n} \cdot \vec{S}_1 \hat{n} \cdot \vec{v}_1 \vec{S}_1 \cdot \vec{v}_1 - \frac{9}{7} \vec{S}_1 \cdot \vec{S}_1 \left( \hat{n} \cdot \vec{v}_1 \right)^2 + \frac{18}{35} \left( \vec{S}_1 \cdot \vec{v}_1 \right)^2 + \frac{9}{35} \vec{S}_1 \cdot \vec{S}_1 \vec{v}_1 \cdot \vec{v}_1 \Big) +$$

$$\frac{1}{r^5} \left( \frac{13}{14} \left( \hat{n} \cdot \vec{S}_1 \cdot \vec{v}_1 \right)^2 - \frac{17}{2} \left( \hat{n} \cdot \vec{S}_1 \right)^2 \left( \hat{n} \cdot \vec{v}_1 \right)^2 + \frac{367}{98} \vec{S}_1 \cdot \vec{S}_1 \left( \hat{n} \cdot \vec{v}_1 \right)^2 + \frac{195}{49} \hat{n} \cdot \vec{S}_1 \hat{n} \cdot \vec{v}_1 \vec{S}_1 \cdot \vec{v}_1 + \right.$$

$$\left. \frac{47}{49} \vec{v}_1 \cdot \vec{v}_1 \left( \hat{n} \cdot \vec{S}_1 \right)^2 - \frac{1143 \left( \vec{S}_1 \cdot \vec{v}_1 \right)^2}{2450} - \frac{1499 \vec{S}_1 \cdot \vec{S}_1 \vec{v}_1 \cdot \vec{v}_1}{2450} \right) \Big\}$$

{DiagS1S1[3, 1, 34],

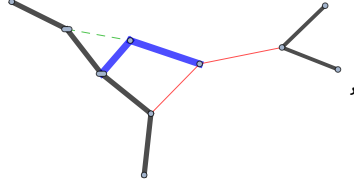

$$\begin{aligned}
 G^3 m_1 m_2 & \left( \frac{1}{r^4} \left( \frac{5}{2} \hat{n} \cdot \vec{a}_1 \left( \hat{n} \cdot \vec{S}_1 \right)^2 - 2 \hat{n} \cdot \vec{S}_1 \hat{n} \cdot \vec{v}_1 \hat{n} \cdot \vec{S}_1 + \frac{23}{50} \vec{S}_1 \cdot \vec{v}_1 \hat{n} \cdot \vec{S}_1 + \frac{17}{10} \vec{S}_1 \cdot \vec{a}_1 \hat{n} \cdot \vec{S}_1 + \frac{29}{25} \hat{n} \cdot \vec{v}_1 \vec{S}_1 \cdot \vec{S}_1 - \right. \right. \\
 & \frac{3}{5} \hat{n} \cdot \vec{a}_1 \vec{S}_1 \cdot \vec{S}_1 + \frac{183}{50} \hat{n} \cdot \vec{S}_1 \vec{S}_1 \cdot \vec{v}_1 \left. \right) + \frac{1}{r^5} \left( -\frac{5}{7} \left( \hat{n} \times \vec{S}_1 \cdot \vec{v}_1 \right)^2 + 3 \left( \hat{n} \cdot \vec{S}_1 \right)^2 \left( \hat{n} \cdot \vec{v}_1 \right)^2 + \frac{2302 \left( \vec{S}_1 \cdot \vec{v}_1 \right)^2}{1225} + \right. \\
 & 7 \left( \hat{n} \cdot \vec{S}_1 \right)^2 \hat{n} \cdot \vec{v}_1 \hat{n} \cdot \vec{v}_2 - \frac{107}{49} \left( \hat{n} \cdot \vec{v}_1 \right)^2 \vec{S}_1 \cdot \vec{S}_1 - \frac{442}{49} \hat{n} \cdot \vec{S}_1 \hat{n} \cdot \vec{v}_1 \vec{S}_1 \cdot \vec{v}_1 + 5 \hat{n} \cdot \vec{S}_1 \hat{n} \cdot \vec{v}_2 \vec{S}_1 \cdot \vec{v}_1 - \\
 & \left. 2 \hat{n} \cdot \vec{S}_1 \hat{n} \cdot \vec{v}_1 \vec{S}_1 \cdot \vec{v}_2 - \vec{S}_1 \cdot \vec{v}_1 \vec{S}_1 \cdot \vec{v}_2 + \frac{5}{49} \left( \hat{n} \cdot \vec{S}_1 \right)^2 \vec{v}_1 \cdot \vec{v}_1 - \frac{109 \vec{S}_1 \cdot \vec{S}_1 \vec{v}_1 \cdot \vec{v}_1}{1225} - \left( \hat{n} \cdot \vec{S}_1 \right)^2 \vec{v}_1 \cdot \vec{v}_2 \right) + \\
 & \left( \frac{6 \hat{n} \cdot \vec{S}_1 \hat{n} \cdot \vec{S}_1 \hat{n} \cdot \vec{v}_1 - \frac{6}{5} \vec{S}_1 \cdot \vec{S}_1 \hat{n} \cdot \vec{v}_1 - \frac{6}{5} \hat{n} \cdot \vec{S}_1 \vec{S}_1 \cdot \vec{v}_1 - \frac{6}{5} \hat{n} \cdot \vec{S}_1 \vec{S}_1 \cdot \vec{v}_1}{r^4} + \frac{1}{r^5} \left( -12 \left( \hat{n} \cdot \vec{v}_1 \right)^2 \left( \hat{n} \cdot \vec{S}_1 \right)^2 + \frac{12}{7} \vec{v}_1 \cdot \vec{v}_1 \right. \right. \\
 & \left. \left( \hat{n} \cdot \vec{S}_1 \right)^2 + \frac{48}{7} \hat{n} \cdot \vec{v}_1 \vec{S}_1 \cdot \vec{v}_1 \hat{n} \cdot \vec{S}_1 - \frac{24}{35} \left( \vec{S}_1 \cdot \vec{v}_1 \right)^2 + \frac{12}{7} \left( \hat{n} \cdot \vec{v}_1 \right)^2 \vec{S}_1 \cdot \vec{S}_1 - \frac{12}{35} \vec{S}_1 \cdot \vec{S}_1 \vec{v}_1 \cdot \vec{v}_1 \right) \log \left( \frac{r}{R_\theta} \right) + \\
 & \frac{1}{\epsilon_d} \left( \frac{-2 \hat{n} \cdot \vec{S}_1 \hat{n} \cdot \vec{S}_1 \hat{n} \cdot \vec{v}_1 + \frac{2}{5} \vec{S}_1 \cdot \vec{S}_1 \hat{n} \cdot \vec{v}_1 + \frac{2}{5} \hat{n} \cdot \vec{S}_1 \vec{S}_1 \cdot \vec{v}_1 + \frac{2}{5} \hat{n} \cdot \vec{S}_1 \vec{S}_1 \cdot \vec{v}_1}{r^4} + \frac{1}{r^5} \left( 4 \left( \hat{n} \cdot \vec{v}_1 \right)^2 \left( \hat{n} \cdot \vec{S}_1 \right)^2 - \right. \right. \\
 & \left. \left. \frac{4}{7} \vec{v}_1 \cdot \vec{v}_1 \left( \hat{n} \cdot \vec{S}_1 \right)^2 - \frac{16}{7} \hat{n} \cdot \vec{v}_1 \vec{S}_1 \cdot \vec{v}_1 \hat{n} \cdot \vec{S}_1 + \frac{8}{35} \left( \vec{S}_1 \cdot \vec{v}_1 \right)^2 - \frac{4}{7} \left( \hat{n} \cdot \vec{v}_1 \right)^2 \vec{S}_1 \cdot \vec{S}_1 + \frac{4}{35} \vec{S}_1 \cdot \vec{S}_1 \vec{v}_1 \cdot \vec{v}_1 \right) \right) \right) \Bigg\}
 \end{aligned}$$

{DiagS1S1[3, 1, 35],

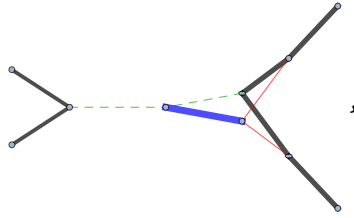

$$\frac{G^3 m_1 m_2 \left( \frac{8}{7} \hat{n} \times \vec{S}_1 \cdot \vec{v}_1 \hat{n} \times \vec{S}_1 \cdot \vec{v}_2 - \frac{24}{7} \vec{S}_1 \cdot \vec{S}_1 \hat{n} \cdot \vec{v}_1 \hat{n} \cdot \vec{v}_2 + \frac{24}{7} \hat{n} \cdot \vec{S}_1 \hat{n} \cdot \vec{v}_2 \vec{S}_1 \cdot \vec{v}_1 + \frac{4}{7} \vec{S}_1 \cdot \vec{v}_1 \vec{S}_1 \cdot \vec{v}_2 - \frac{4}{7} \vec{S}_1 \cdot \vec{S}_1 \vec{v}_1 \cdot \vec{v}_2 \right)}{r^5} \Bigg\}$$

{DiagS1S1[3, 1, 36],

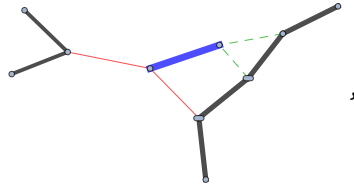

$$\frac{G^3 m_1 m_2 \left( -\frac{60}{7} \left( \hat{n} \times \vec{S}_1 \cdot \vec{v}_1 \right)^2 + \frac{20}{7} \vec{S}_1 \cdot \vec{S}_1 \left( \hat{n} \cdot \vec{v}_1 \right)^2 - \frac{20}{7} \hat{n} \cdot \vec{S}_1 \hat{n} \cdot \vec{v}_1 \vec{S}_1 \cdot \vec{v}_1 - \frac{4}{7} \left( \vec{S}_1 \cdot \vec{v}_1 \right)^2 + \frac{4}{7} \vec{S}_1 \cdot \vec{S}_1 \vec{v}_1 \cdot \vec{v}_1 \right)}{r^5}$$

{DiagS1S1[3, 1, 37],

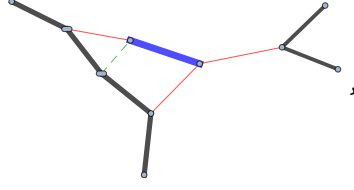

$$G^3 m_1 m_2 \left( \frac{-\frac{14}{5} \vec{S}_1 \cdot \vec{a}_1 \hat{n} \cdot \vec{S}_1 + \frac{14}{5} \vec{S}_1 \cdot \vec{S}_1 \hat{n} \cdot \vec{a}_1 + \frac{6}{5} \hat{n} \cdot \vec{S}_1 \vec{S}_1 \cdot \vec{v}_1 + \frac{8}{5} \vec{S}_1 \cdot \vec{S}_1 \hat{n} \cdot \vec{v}_1 - \frac{14}{5} \hat{n} \cdot \vec{S}_1 \vec{S}_1 \cdot \vec{v}_1}{r^4} + \right.$$

$$\left. \frac{\frac{4}{7} \left( \hat{n} \times \vec{S}_1 \cdot \vec{v}_1 \right)^2 - \frac{20}{7} \vec{S}_1 \cdot \vec{S}_1 \left( \hat{n} \cdot \vec{v}_1 \right)^2 + \frac{20}{7} \hat{n} \cdot \vec{S}_1 \hat{n} \cdot \vec{v}_1 \vec{S}_1 \cdot \vec{v}_1 - \frac{36}{35} \left( \vec{S}_1 \cdot \vec{v}_1 \right)^2 + \frac{36}{35} \vec{S}_1 \cdot \vec{S}_1 \vec{v}_1 \cdot \vec{v}_1}{r^5} \right\}$$

{DiagS1S1[3, 1, 38],

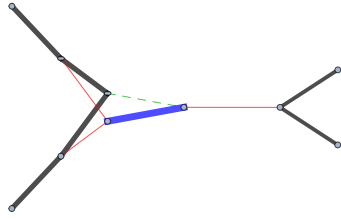

,  $G^3 m_1 m_2$

$$\left( \frac{1}{r^5} \left( -\frac{18}{7} \left( \hat{n} \times \vec{S}_1 \cdot \vec{v}_1 \right)^2 - \frac{24}{7} \vec{S}_1 \cdot \vec{S}_1 \left( \hat{n} \cdot \vec{v}_1 \right)^2 + 6 \vec{S}_1 \cdot \vec{S}_1 \hat{n} \cdot \vec{v}_1 \hat{n} \cdot \vec{v}_2 + \frac{24}{7} \hat{n} \cdot \vec{S}_1 \hat{n} \cdot \vec{v}_1 \vec{S}_1 \cdot \vec{v}_1 - 6 \hat{n} \cdot \vec{S}_1 \hat{n} \cdot \vec{v}_2 \vec{S}_1 \cdot \vec{v}_1 - \right.$$

$$\left. \frac{6}{5} \left( \vec{S}_1 \cdot \vec{v}_1 \right)^2 + \frac{6}{5} \vec{S}_1 \cdot \vec{v}_1 \vec{S}_1 \cdot \vec{v}_2 + \frac{6}{5} \vec{S}_1 \cdot \vec{S}_1 \vec{v}_1 \cdot \vec{v}_1 - \frac{6}{5} \vec{S}_1 \cdot \vec{S}_1 \vec{v}_1 \cdot \vec{v}_2 \right) + \frac{\frac{6}{5} \vec{S}_1 \cdot \vec{S}_1 \hat{n} \cdot \vec{v}_1 - \frac{6}{5} \hat{n} \cdot \vec{S}_1 \vec{S}_1 \cdot \vec{v}_1}{r^4} \right\}$$

{DiagS1S1[3, 1, 39],

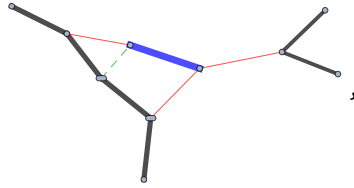

$$G^3 m_1 m_2 \left( \frac{6 \left( \hat{n} \times \vec{S}_1 \cdot \vec{v}_1 \right)^2 + 2 \left( \vec{S}_1 \cdot \vec{v}_1 \right)^2 - 2 \vec{S}_1 \cdot \vec{S}_1 \vec{v}_1 \cdot \vec{v}_1}{r^5} + \frac{2 \vec{S}_1 \cdot \vec{S}_1 \hat{n} \cdot \vec{v}_1 - 2 \hat{n} \cdot \vec{S}_1 \vec{S}_1 \cdot \vec{v}_1}{r^4} \right\}$$

{DiagS1S1[3, 1, 40],

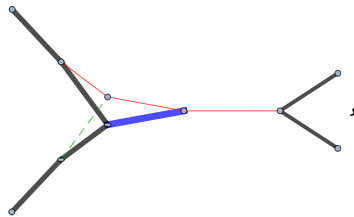

$$\frac{G^3 m_1 m_2 \left( -\frac{2}{7} \left( \hat{n} \times \vec{S}_1 \cdot \vec{v}_1 \right)^2 + \frac{11}{14} \vec{S}_1 \cdot \vec{S}_1 \left( \hat{n} \cdot \vec{v}_1 \right)^2 - \frac{11}{14} \hat{n} \cdot \vec{S}_1 \hat{n} \cdot \vec{v}_1 \vec{S}_1 \cdot \vec{v}_1 + \frac{1}{10} \left( \vec{S}_1 \cdot \vec{v}_1 \right)^2 - \frac{1}{10} \vec{S}_1 \cdot \vec{S}_1 \vec{v}_1 \cdot \vec{v}_1 \right)}{r^5}$$

$\{\text{DiagS1S1}[3, 1, 41],$

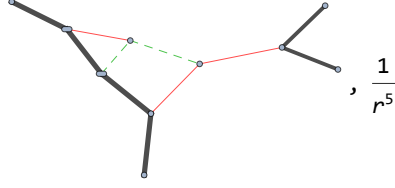

$, \frac{1}{r^5}$

$$G^3 m_1 m_2 \left( \frac{2}{7} \vec{S}_1 \cdot \vec{S}_1 (\hat{n} \cdot \vec{v}_1)^2 + 2 \vec{S}_1 \cdot \vec{S}_1 \hat{n} \cdot \vec{v}_2 \hat{n} \cdot \vec{v}_1 - \frac{2}{7} \hat{n} \cdot \vec{S}_1 \hat{n} \cdot \vec{v}_1 \vec{S}_1 \cdot \vec{v}_1 - \right. \\ \left. 2 \hat{n} \cdot \vec{S}_1 \hat{n} \cdot \vec{v}_2 \vec{S}_1 \cdot \vec{v}_1 - \frac{6}{35} (\vec{S}_1 \cdot \vec{v}_1)^2 + \frac{2}{5} \vec{S}_1 \cdot \vec{v}_1 \vec{S}_1 \cdot \vec{v}_2 + \frac{6}{35} \vec{S}_1 \cdot \vec{S}_1 \vec{v}_1 \cdot \vec{v}_1 - \frac{2}{5} \vec{S}_1 \cdot \vec{S}_1 \vec{v}_1 \cdot \vec{v}_2 \right) \}$$

$\{\text{DiagS1S1}[3, 1, 42],$

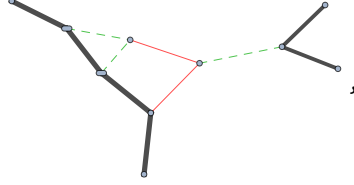

,

$$G^3 m_1 m_2 \left( \frac{-\frac{16}{49} \hat{n} \cdot \vec{S}_1 \hat{n} \cdot \vec{S}_1 \hat{n} \cdot \vec{v}_2 - \frac{4 \vec{S}_1 \cdot \vec{S}_1 \hat{n} \cdot \vec{v}_2}{1225} - \frac{144 \hat{n} \cdot \vec{S}_1 \vec{S}_1 \cdot \vec{v}_2}{1225} - \frac{144 \hat{n} \cdot \vec{S}_1 \vec{S}_1 \cdot \vec{v}_2}{1225}}{r^4} + \right. \\ \frac{1}{r^5} \left( \frac{8}{3} \hat{n} \cdot \vec{v}_1 \hat{n} \cdot \vec{v}_2 (\hat{n} \cdot \vec{S}_1)^2 + \frac{8}{49} \vec{v}_1 \cdot \vec{v}_2 (\hat{n} \cdot \vec{S}_1)^2 - \frac{12}{49} \hat{n} \cdot \vec{v}_2 \vec{S}_1 \cdot \vec{v}_1 \hat{n} \cdot \vec{S}_1 - \right. \\ \left. \frac{12}{49} \hat{n} \cdot \vec{v}_1 \vec{S}_1 \cdot \vec{v}_2 \hat{n} \cdot \vec{S}_1 - \frac{32}{147} \hat{n} \cdot \vec{v}_1 \hat{n} \cdot \vec{v}_2 \vec{S}_1 \cdot \vec{S}_1 - \frac{436 \vec{S}_1 \cdot \vec{v}_1 \vec{S}_1 \cdot \vec{v}_2}{3675} - \frac{148 \vec{S}_1 \cdot \vec{S}_1 \vec{v}_1 \cdot \vec{v}_2}{3675} \right) + \\ \left( \frac{\frac{12}{7} \hat{n} \cdot \vec{S}_1 \hat{n} \cdot \vec{S}_1 \hat{n} \cdot \vec{v}_2 - \frac{12}{35} \vec{S}_1 \cdot \vec{S}_1 \hat{n} \cdot \vec{v}_2 - \frac{12}{35} \hat{n} \cdot \vec{S}_1 \vec{S}_1 \cdot \vec{v}_2 - \frac{12}{35} \hat{n} \cdot \vec{S}_1 \vec{S}_1 \cdot \vec{v}_2}{r^4} + \frac{1}{r^5} \right. \\ \left( -8 \hat{n} \cdot \vec{v}_1 \hat{n} \cdot \vec{v}_2 (\hat{n} \cdot \vec{S}_1)^2 + \frac{8}{7} \vec{v}_1 \cdot \vec{v}_2 (\hat{n} \cdot \vec{S}_1)^2 + \frac{16}{7} \hat{n} \cdot \vec{v}_2 \vec{S}_1 \cdot \vec{v}_1 \hat{n} \cdot \vec{S}_1 + \frac{16}{7} \hat{n} \cdot \vec{v}_1 \vec{S}_1 \cdot \vec{v}_2 \hat{n} \cdot \vec{S}_1 + \right. \\ \left. \frac{8}{7} \hat{n} \cdot \vec{v}_1 \hat{n} \cdot \vec{v}_2 \vec{S}_1 \cdot \vec{S}_1 - \frac{16}{35} \vec{S}_1 \cdot \vec{v}_1 \vec{S}_1 \cdot \vec{v}_2 - \frac{8}{35} \vec{S}_1 \cdot \vec{S}_1 \vec{v}_1 \cdot \vec{v}_2 \right) \log\left(\frac{r}{R_0}\right) + \\ \frac{1}{\epsilon_d} \left( \frac{-\frac{4}{7} \hat{n} \cdot \vec{S}_1 \hat{n} \cdot \vec{S}_1 \hat{n} \cdot \vec{v}_2 + \frac{4}{35} \vec{S}_1 \cdot \vec{S}_1 \hat{n} \cdot \vec{v}_2 + \frac{4}{35} \hat{n} \cdot \vec{S}_1 \vec{S}_1 \cdot \vec{v}_2 + \frac{4}{35} \hat{n} \cdot \vec{S}_1 \vec{S}_1 \cdot \vec{v}_2}{r^4} + \frac{1}{r^5} \right. \\ \left( \frac{8}{3} \hat{n} \cdot \vec{v}_1 \hat{n} \cdot \vec{v}_2 (\hat{n} \cdot \vec{S}_1)^2 - \frac{8}{21} \vec{v}_1 \cdot \vec{v}_2 (\hat{n} \cdot \vec{S}_1)^2 - \frac{16}{21} \hat{n} \cdot \vec{v}_2 \vec{S}_1 \cdot \vec{v}_1 \hat{n} \cdot \vec{S}_1 - \right. \\ \left. \frac{16}{21} \hat{n} \cdot \vec{v}_1 \vec{S}_1 \cdot \vec{v}_2 \hat{n} \cdot \vec{S}_1 - \frac{8}{21} \hat{n} \cdot \vec{v}_1 \hat{n} \cdot \vec{v}_2 \vec{S}_1 \cdot \vec{S}_1 + \frac{16}{105} \vec{S}_1 \cdot \vec{v}_1 \vec{S}_1 \cdot \vec{v}_2 + \frac{8}{105} \vec{S}_1 \cdot \vec{S}_1 \vec{v}_1 \cdot \vec{v}_2 \right) \left. \right) \left. \right) \}$$

$\{\text{DiagS1S1}[3, 1, 43],$

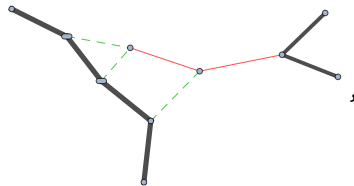

,

$$\begin{aligned}
& G^3 m_1 m_2 \left( \frac{\frac{12}{25} \hat{n} \cdot \vec{S}_1 \vec{S}_1 \cdot \vec{v}_1 + \frac{12}{25} \hat{n} \cdot \vec{v}_1 \vec{S}_1 \cdot \vec{S}_1 + \frac{12}{25} \hat{n} \cdot \vec{S}_1 \vec{S}_1 \cdot \vec{v}_1}{r^4} + \frac{1}{r^5} \right. \\
& \left( -4 (\hat{n} \cdot \vec{v}_1)^2 (\hat{n} \cdot \vec{S}_1)^2 - 4 \hat{n} \cdot \vec{v}_1 \hat{n} \cdot \vec{v}_2 (\hat{n} \cdot \vec{S}_1)^2 - \frac{8}{49} \vec{v}_1 \cdot \vec{v}_1 (\hat{n} \cdot \vec{S}_1)^2 - \frac{8}{49} \vec{v}_1 \cdot \vec{v}_2 (\hat{n} \cdot \vec{S}_1)^2 - \right. \\
& \frac{4}{49} \hat{n} \cdot \vec{v}_1 \vec{S}_1 \cdot \vec{v}_1 \hat{n} \cdot \vec{S}_1 + \frac{12}{49} \hat{n} \cdot \vec{v}_2 \vec{S}_1 \cdot \vec{v}_1 \hat{n} \cdot \vec{S}_1 - \frac{16}{49} \hat{n} \cdot \vec{v}_1 \vec{S}_1 \cdot \vec{v}_2 \hat{n} \cdot \vec{S}_1 + \frac{444 (\vec{S}_1 \cdot \vec{v}_1)^2}{1225} - \\
& \left. \frac{8}{49} (\hat{n} \cdot \vec{v}_1)^2 \vec{S}_1 \cdot \vec{S}_1 - \frac{8}{49} \hat{n} \cdot \vec{v}_1 \hat{n} \cdot \vec{v}_2 \vec{S}_1 \cdot \vec{S}_1 + \frac{444 \vec{S}_1 \cdot \vec{v}_1 \vec{S}_1 \cdot \vec{v}_2}{1225} + \frac{292 \vec{S}_1 \cdot \vec{S}_1 \vec{v}_1 \cdot \vec{v}_1}{1225} + \frac{292 \vec{S}_1 \cdot \vec{S}_1 \vec{v}_1 \cdot \vec{v}_2}{1225} \right) + \\
& \left( \frac{-12 \hat{n} \cdot \vec{S}_1 \hat{n} \cdot \vec{S}_1 \hat{n} \cdot \vec{v}_1 + \frac{12}{5} \vec{S}_1 \cdot \vec{S}_1 \hat{n} \cdot \vec{v}_1 + \frac{12}{5} \hat{n} \cdot \vec{S}_1 \vec{S}_1 \cdot \vec{v}_1 + \frac{12}{5} \hat{n} \cdot \vec{S}_1 \vec{S}_1 \cdot \vec{v}_1}{r^4} + \frac{1}{r^5} \right. \\
& \left( 36 (\hat{n} \cdot \vec{v}_1)^2 (\hat{n} \cdot \vec{S}_1)^2 + 36 \hat{n} \cdot \vec{v}_1 \hat{n} \cdot \vec{v}_2 (\hat{n} \cdot \vec{S}_1)^2 - \frac{36}{7} \vec{v}_1 \cdot \vec{v}_1 (\hat{n} \cdot \vec{S}_1)^2 - \frac{36}{7} \vec{v}_1 \cdot \vec{v}_2 (\hat{n} \cdot \vec{S}_1)^2 - \right. \\
& \frac{144}{7} \hat{n} \cdot \vec{v}_1 \vec{S}_1 \cdot \vec{v}_1 \hat{n} \cdot \vec{S}_1 - \frac{72}{7} \hat{n} \cdot \vec{v}_2 \vec{S}_1 \cdot \vec{v}_1 \hat{n} \cdot \vec{S}_1 - \frac{72}{7} \hat{n} \cdot \vec{v}_1 \vec{S}_1 \cdot \vec{v}_2 \hat{n} \cdot \vec{S}_1 + \frac{72}{35} (\vec{S}_1 \cdot \vec{v}_1)^2 - \\
& \left. \frac{36}{7} (\hat{n} \cdot \vec{v}_1)^2 \vec{S}_1 \cdot \vec{S}_1 - \frac{36}{7} \hat{n} \cdot \vec{v}_1 \hat{n} \cdot \vec{v}_2 \vec{S}_1 \cdot \vec{S}_1 + \frac{72}{35} \vec{S}_1 \cdot \vec{v}_1 \vec{S}_1 \cdot \vec{v}_2 + \frac{36}{35} \vec{S}_1 \cdot \vec{S}_1 \vec{v}_1 \cdot \vec{v}_1 + \frac{36}{35} \vec{S}_1 \cdot \vec{S}_1 \vec{v}_1 \cdot \vec{v}_2 \right) \left. \right) \\
& \log \left( \frac{r}{R_\theta} \right) + \frac{1}{\epsilon_d} \left( \frac{4 \hat{n} \cdot \vec{S}_1 \hat{n} \cdot \vec{S}_1 \hat{n} \cdot \vec{v}_1 - \frac{4}{5} \vec{S}_1 \cdot \vec{S}_1 \hat{n} \cdot \vec{v}_1 - \frac{4}{5} \hat{n} \cdot \vec{S}_1 \vec{S}_1 \cdot \vec{v}_1 - \frac{4}{5} \hat{n} \cdot \vec{S}_1 \vec{S}_1 \cdot \vec{v}_1}{r^4} + \frac{1}{r^5} \right. \\
& \left( -12 (\hat{n} \cdot \vec{v}_1)^2 (\hat{n} \cdot \vec{S}_1)^2 - 12 \hat{n} \cdot \vec{v}_1 \hat{n} \cdot \vec{v}_2 (\hat{n} \cdot \vec{S}_1)^2 + \frac{12}{7} \vec{v}_1 \cdot \vec{v}_1 (\hat{n} \cdot \vec{S}_1)^2 + \frac{12}{7} \vec{v}_1 \cdot \vec{v}_2 (\hat{n} \cdot \vec{S}_1)^2 + \right. \\
& \frac{48}{7} \hat{n} \cdot \vec{v}_1 \vec{S}_1 \cdot \vec{v}_1 \hat{n} \cdot \vec{S}_1 + \frac{24}{7} \hat{n} \cdot \vec{v}_2 \vec{S}_1 \cdot \vec{v}_1 \hat{n} \cdot \vec{S}_1 + \frac{24}{7} \hat{n} \cdot \vec{v}_1 \vec{S}_1 \cdot \vec{v}_2 \hat{n} \cdot \vec{S}_1 - \frac{24}{35} (\vec{S}_1 \cdot \vec{v}_1)^2 + \\
& \left. \frac{12}{7} (\hat{n} \cdot \vec{v}_1)^2 \vec{S}_1 \cdot \vec{S}_1 + \frac{12}{7} \hat{n} \cdot \vec{v}_1 \hat{n} \cdot \vec{v}_2 \vec{S}_1 \cdot \vec{S}_1 - \frac{24}{35} \vec{S}_1 \cdot \vec{v}_1 \vec{S}_1 \cdot \vec{v}_2 - \frac{12}{35} \vec{S}_1 \cdot \vec{S}_1 \vec{v}_1 \cdot \vec{v}_1 - \frac{12}{35} \vec{S}_1 \cdot \vec{S}_1 \vec{v}_1 \cdot \vec{v}_2 \right) \left. \right) \left. \right\}
\end{aligned}$$

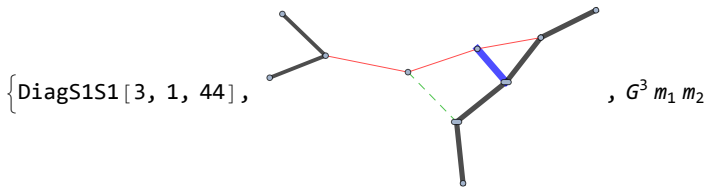

$$\left( \frac{\frac{1}{10} \vec{S}_1 \cdot \vec{a}_1 \hat{n} \cdot \vec{S}_1 - \frac{1}{10} \vec{S}_1 \cdot \vec{S}_1 \hat{n} \cdot \vec{a}_1 - \frac{1}{10} \vec{S}_1 \cdot \vec{S}_1 \hat{n} \cdot \vec{v}_1 + \frac{1}{10} \hat{n} \cdot \vec{S}_1 \vec{S}_1 \cdot \vec{v}_1}{r^4} + \frac{1}{r^5} \left( -\frac{2}{7} (\hat{n} \times \vec{S}_1 \cdot \vec{v}_1)^2 + \frac{2}{7} \vec{S}_1 \cdot \vec{S}_1 (\hat{n} \cdot \vec{v}_1)^2 + \right. \right.$$

$$\left. \left. \frac{1}{2} \vec{S}_1 \cdot \vec{S}_1 \hat{n} \cdot \vec{v}_1 \hat{n} \cdot \vec{v}_2 - \frac{2}{7} \hat{n} \cdot \vec{S}_1 \hat{n} \cdot \vec{v}_1 \vec{S}_1 \cdot \vec{v}_1 - \frac{1}{2} \hat{n} \cdot \vec{S}_1 \hat{n} \cdot \vec{v}_2 \vec{S}_1 \cdot \vec{v}_1 + \frac{1}{10} \vec{S}_1 \cdot \vec{v}_1 \vec{S}_1 \cdot \vec{v}_2 - \frac{1}{10} \vec{S}_1 \cdot \vec{S}_1 \vec{v}_1 \cdot \vec{v}_2 \right) \right\}$$

{DiagS1S1[3, 1, 45],

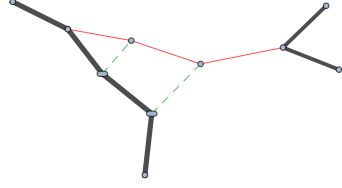

,  $G^3 m_1 m_2$

$$\left( \frac{-\frac{1}{10} \vec{S}_1 \cdot \vec{a}_1 \hat{n} \cdot \vec{S}_1 + \frac{1}{10} \vec{S}_1 \cdot \vec{S}_1 \hat{n} \cdot \vec{a}_1 + \frac{1}{10} \vec{S}_1 \cdot \vec{S}_1 \hat{n} \cdot \vec{v}_1 - \frac{1}{10} \hat{n} \cdot \vec{S}_1 \vec{S}_1 \cdot \vec{v}_1}{r^4} + \frac{1}{r^5} \left( \frac{2}{7} (\hat{n} \times \vec{S}_1 \cdot \vec{v}_1)^2 - \frac{2}{7} \vec{S}_1 \cdot \vec{S}_1 (\hat{n} \cdot \vec{v}_1)^2 - \right. \right.$$

$$\left. \frac{1}{2} \vec{S}_1 \cdot \vec{S}_1 \hat{n} \cdot \vec{v}_1 \hat{n} \cdot \vec{v}_2 + \frac{2}{7} \hat{n} \cdot \vec{S}_1 \hat{n} \cdot \vec{v}_1 \vec{S}_1 \cdot \vec{v}_1 + \frac{1}{2} \hat{n} \cdot \vec{S}_1 \hat{n} \cdot \vec{v}_2 \vec{S}_1 \cdot \vec{v}_1 - \frac{1}{10} \vec{S}_1 \cdot \vec{v}_1 \vec{S}_1 \cdot \vec{v}_2 + \frac{1}{10} \vec{S}_1 \cdot \vec{S}_1 \vec{v}_1 \cdot \vec{v}_2 \right) \Bigg\}$$

{DiagS1S1[3, 1, 46],

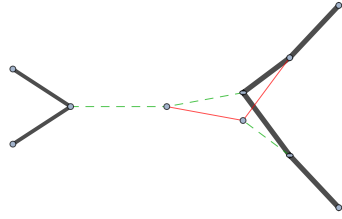

,

$$\frac{G^3 m_1 m_2 \left( -\frac{2}{7} \hat{n} \times \vec{S}_1 \cdot \vec{v}_1 \hat{n} \times \vec{S}_1 \cdot \vec{v}_2 + \frac{6}{7} \vec{S}_1 \cdot \vec{S}_1 \hat{n} \cdot \vec{v}_1 \hat{n} \cdot \vec{v}_2 - \frac{6}{7} \hat{n} \cdot \vec{S}_1 \hat{n} \cdot \vec{v}_2 \vec{S}_1 \cdot \vec{v}_1 + \frac{16}{35} \vec{S}_1 \cdot \vec{v}_1 \vec{S}_1 \cdot \vec{v}_2 - \frac{16}{35} \vec{S}_1 \cdot \vec{S}_1 \vec{v}_1 \cdot \vec{v}_2 \right)}{r^5} \Bigg\}$$

{DiagS1S1[3, 1, 47],

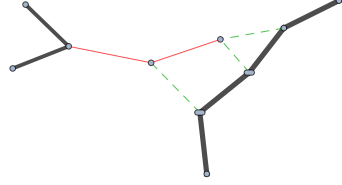

,

$$G^3 m_1 m_2 \left( \frac{-\frac{2}{5} \vec{S}_1 \cdot \vec{a}_1 \hat{n} \cdot \vec{S}_1 + \frac{2}{5} \vec{S}_1 \cdot \vec{S}_1 \hat{n} \cdot \vec{a}_1 + \frac{2}{5} \vec{S}_1 \cdot \vec{S}_1 \hat{n} \cdot \vec{v}_1 - \frac{2}{5} \hat{n} \cdot \vec{S}_1 \vec{S}_1 \cdot \vec{v}_1}{r^4} + \frac{1}{r^5} \left( \frac{8}{7} (\hat{n} \times \vec{S}_1 \cdot \vec{v}_1)^2 - \frac{8}{7} \vec{S}_1 \cdot \vec{S}_1 (\hat{n} \cdot \vec{v}_1)^2 - \right. \right.$$

$$\left. 2 \vec{S}_1 \cdot \vec{S}_1 \hat{n} \cdot \vec{v}_1 \hat{n} \cdot \vec{v}_2 + \frac{8}{7} \hat{n} \cdot \vec{S}_1 \hat{n} \cdot \vec{v}_1 \vec{S}_1 \cdot \vec{v}_1 + 2 \hat{n} \cdot \vec{S}_1 \hat{n} \cdot \vec{v}_2 \vec{S}_1 \cdot \vec{v}_1 - \frac{2}{5} \vec{S}_1 \cdot \vec{v}_1 \vec{S}_1 \cdot \vec{v}_2 + \frac{2}{5} \vec{S}_1 \cdot \vec{S}_1 \vec{v}_1 \cdot \vec{v}_2 \right) \Bigg\}$$

{DiagS1S1[3, 1, 48],

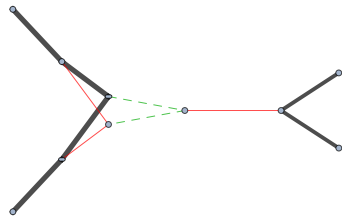

,

$$G^3 m_1 m_2 \left( \frac{\frac{2}{5} \vec{S}_1 \cdot \vec{a}_1 \hat{n} \cdot \vec{S}_1 - \frac{2}{5} \vec{S}_1 \cdot \vec{S}_1 \hat{n} \cdot \vec{a}_1 - \frac{2}{5} \vec{S}_1 \cdot \vec{S}_1 \hat{n} \cdot \vec{v}_1 + \frac{2}{5} \hat{n} \cdot \vec{S}_1 \vec{S}_1 \cdot \vec{v}_1}{r^4} + \right.$$

$$\left. \frac{-\frac{2}{7} \left( \hat{n} \times \vec{S}_1 \cdot \vec{v}_1 \right)^2 + \frac{6}{7} \vec{S}_1 \cdot \vec{S}_1 \left( \hat{n} \cdot \vec{v}_1 \right)^2 - \frac{6}{7} \hat{n} \cdot \vec{S}_1 \hat{n} \cdot \vec{v}_1 \vec{S}_1 \cdot \vec{v}_1 + \frac{16}{35} \left( \vec{S}_1 \cdot \vec{v}_1 \right)^2 - \frac{16}{35} \vec{S}_1 \cdot \vec{S}_1 \vec{v}_1 \cdot \vec{v}_1}{r^5} \right\}$$

{DiagS1S1[3, 1, 49],

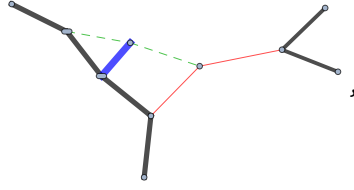

$$\begin{aligned} G^3 m_1 m_2 \left( \frac{1}{r^5 \in_d} \left( \left( \hat{n} \cdot \vec{v}_1 \right)^2 \left( \hat{n} \cdot \vec{S}_1 \right)^2 + \hat{n} \cdot \vec{v}_1 \hat{n} \cdot \vec{v}_2 \left( \hat{n} \cdot \vec{S}_1 \right)^2 - \frac{1}{7} \vec{v}_1 \cdot \vec{v}_1 \left( \hat{n} \cdot \vec{S}_1 \right)^2 - \frac{1}{7} \vec{v}_1 \cdot \vec{v}_2 \left( \hat{n} \cdot \vec{S}_1 \right)^2 - \right. \right. \\ \left. \frac{4}{7} \hat{n} \cdot \vec{v}_1 \vec{S}_1 \cdot \vec{v}_1 \hat{n} \cdot \vec{S}_1 - \frac{2}{7} \hat{n} \cdot \vec{v}_2 \vec{S}_1 \cdot \vec{v}_1 \hat{n} \cdot \vec{S}_1 - \frac{2}{7} \hat{n} \cdot \vec{v}_1 \vec{S}_1 \cdot \vec{v}_2 \hat{n} \cdot \vec{S}_1 + \frac{2}{35} \left( \vec{S}_1 \cdot \vec{v}_1 \right)^2 - \right. \\ \left. \frac{1}{7} \left( \hat{n} \cdot \vec{v}_1 \right)^2 \vec{S}_1 \cdot \vec{S}_1 - \frac{1}{7} \hat{n} \cdot \vec{v}_1 \hat{n} \cdot \vec{v}_2 \vec{S}_1 \cdot \vec{S}_1 + \frac{2}{35} \vec{S}_1 \cdot \vec{v}_1 \vec{S}_1 \cdot \vec{v}_2 + \frac{1}{35} \vec{S}_1 \cdot \vec{S}_1 \vec{v}_1 \cdot \vec{v}_1 + \frac{1}{35} \vec{S}_1 \cdot \vec{S}_1 \vec{v}_1 \cdot \vec{v}_2 \right) + \\ \left. \frac{1}{r^5} \left( \frac{7}{2} \left( \hat{n} \cdot \vec{v}_1 \right)^2 \left( \hat{n} \cdot \vec{S}_1 \right)^2 + \frac{7}{2} \hat{n} \cdot \vec{v}_1 \hat{n} \cdot \vec{v}_2 \left( \hat{n} \cdot \vec{S}_1 \right)^2 - \frac{15}{98} \vec{v}_1 \cdot \vec{v}_1 \left( \hat{n} \cdot \vec{S}_1 \right)^2 - \frac{43}{98} \vec{v}_1 \cdot \vec{v}_2 \left( \hat{n} \cdot \vec{S}_1 \right)^2 - \right. \right. \\ \left. \frac{123}{98} \hat{n} \cdot \vec{v}_1 \vec{S}_1 \cdot \vec{v}_1 \hat{n} \cdot \vec{S}_1 + \frac{89}{98} \hat{n} \cdot \vec{v}_2 \vec{S}_1 \cdot \vec{v}_1 \hat{n} \cdot \vec{S}_1 - \frac{43}{49} \hat{n} \cdot \vec{v}_1 \vec{S}_1 \cdot \vec{v}_2 \hat{n} \cdot \vec{S}_1 + \frac{521 \left( \vec{S}_1 \cdot \vec{v}_1 \right)^2}{2450} - \right. \\ \left. \frac{102}{49} \left( \hat{n} \cdot \vec{v}_1 \right)^2 \vec{S}_1 \cdot \vec{S}_1 - \frac{193}{49} \hat{n} \cdot \vec{v}_1 \hat{n} \cdot \vec{v}_2 \vec{S}_1 \cdot \vec{S}_1 - \frac{529 \vec{S}_1 \cdot \vec{v}_1 \vec{S}_1 \cdot \vec{v}_2}{2450} + \frac{69 \vec{S}_1 \cdot \vec{S}_1 \vec{v}_1 \cdot \vec{v}_1}{1225} + \frac{944 \vec{S}_1 \cdot \vec{S}_1 \vec{v}_1 \cdot \vec{v}_2}{1225} \right) + \\ \left. \frac{1}{r^5} \left( -3 \left( \hat{n} \cdot \vec{v}_1 \right)^2 \left( \hat{n} \cdot \vec{S}_1 \right)^2 - 3 \hat{n} \cdot \vec{v}_1 \hat{n} \cdot \vec{v}_2 \left( \hat{n} \cdot \vec{S}_1 \right)^2 + \frac{3}{7} \vec{v}_1 \cdot \vec{v}_1 \left( \hat{n} \cdot \vec{S}_1 \right)^2 + \frac{3}{7} \vec{v}_1 \cdot \vec{v}_2 \left( \hat{n} \cdot \vec{S}_1 \right)^2 + \right. \\ \left. \frac{12}{7} \hat{n} \cdot \vec{v}_1 \vec{S}_1 \cdot \vec{v}_1 \hat{n} \cdot \vec{S}_1 + \frac{6}{7} \hat{n} \cdot \vec{v}_2 \vec{S}_1 \cdot \vec{v}_1 \hat{n} \cdot \vec{S}_1 + \frac{6}{7} \hat{n} \cdot \vec{v}_1 \vec{S}_1 \cdot \vec{v}_2 \hat{n} \cdot \vec{S}_1 - \frac{6}{35} \left( \vec{S}_1 \cdot \vec{v}_1 \right)^2 + \frac{3}{7} \left( \hat{n} \cdot \vec{v}_1 \right)^2 \vec{S}_1 \cdot \vec{S}_1 + \right. \\ \left. \frac{3}{7} \hat{n} \cdot \vec{v}_1 \hat{n} \cdot \vec{v}_2 \vec{S}_1 \cdot \vec{S}_1 - \frac{6}{35} \vec{S}_1 \cdot \vec{v}_1 \vec{S}_1 \cdot \vec{v}_2 - \frac{3}{35} \vec{S}_1 \cdot \vec{S}_1 \vec{v}_1 \cdot \vec{v}_1 - \frac{3}{35} \vec{S}_1 \cdot \vec{S}_1 \vec{v}_1 \cdot \vec{v}_2 \right) \log \left( \frac{r}{R_\theta} \right) \right) \Bigg\} \end{aligned}$$

{DiagS1S1[3, 1, 50],

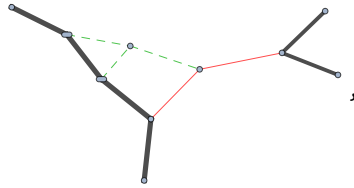

$$\begin{aligned} G^3 m_1 m_2 \left( \frac{1}{r^4} \left( - \left( \hat{n} \cdot \vec{a}_1 \right) \left( \hat{n} \cdot \vec{S}_1 \right)^2 - \hat{n} \cdot \vec{a}_2 \left( \hat{n} \cdot \vec{S}_1 \right)^2 + \frac{101}{98} \hat{n} \cdot \vec{S}_1 \hat{n} \cdot \vec{v}_1 \hat{n} \cdot \vec{S}_1 + \frac{7}{2} \hat{n} \cdot \vec{S}_1 \hat{n} \cdot \vec{v}_2 \hat{n} \cdot \vec{S}_1 - \right. \right. \\ \left. \frac{169 \vec{S}_1 \cdot \vec{v}_1 \hat{n} \cdot \vec{S}_1}{2450} - \frac{29}{50} \vec{S}_1 \cdot \vec{v}_2 \hat{n} \cdot \vec{S}_1 + \frac{9}{50} \vec{S}_1 \cdot \vec{a}_1 \hat{n} \cdot \vec{S}_1 + \frac{7}{25} \vec{S}_1 \cdot \vec{a}_2 \hat{n} \cdot \vec{S}_1 - \frac{379 \hat{n} \cdot \vec{v}_1 \vec{S}_1 \cdot \vec{S}_1}{2450} - \right. \\ \left. \frac{29}{50} \hat{n} \cdot \vec{v}_2 \vec{S}_1 \cdot \vec{S}_1 + \frac{27}{50} \hat{n} \cdot \vec{a}_1 \vec{S}_1 \cdot \vec{S}_1 + \frac{16}{25} \hat{n} \cdot \vec{a}_2 \vec{S}_1 \cdot \vec{S}_1 - \frac{169 \hat{n} \cdot \vec{S}_1 \vec{S}_1 \cdot \vec{v}_1}{2450} - \frac{29}{50} \hat{n} \cdot \vec{S}_1 \vec{S}_1 \cdot \vec{v}_2 \right) + \frac{1}{r^5} \\ \left( \frac{1}{7} \left( \hat{n} \times \vec{S}_1 \cdot \vec{v}_1 \right)^2 + \frac{71}{48} \left( \hat{n} \cdot \vec{S}_1 \right)^2 \left( \hat{n} \cdot \vec{v}_1 \right)^2 - \frac{17}{2} \left( \hat{n} \cdot \vec{S}_1 \right)^2 \left( \hat{n} \cdot \vec{v}_2 \right)^2 - \frac{71 \left( \vec{S}_1 \cdot \vec{v}_1 \right)^2}{29400} - \frac{7}{25} \left( \vec{S}_1 \cdot \vec{v}_2 \right)^2 - \right. \end{aligned}$$

$$\begin{aligned}
& 13 \left( \hat{n} \cdot \vec{S}_1 \right)^2 \hat{n} \cdot \vec{v}_1 \hat{n} \cdot \vec{v}_2 - \frac{2657 \left( \hat{n} \cdot \vec{v}_1 \right)^2 \vec{S}_1 \cdot \vec{S}_1}{2352} + \frac{7}{2} \left( \hat{n} \cdot \vec{v}_2 \right)^2 \vec{S}_1 \cdot \vec{S}_1 + \frac{305}{98} \hat{n} \cdot \vec{v}_1 \hat{n} \cdot \vec{v}_2 \vec{S}_1 \cdot \vec{S}_1 - \\
& \frac{179}{588} \hat{n} \cdot \vec{S}_1 \hat{n} \cdot \vec{v}_1 \vec{S}_1 \cdot \vec{v}_1 + \frac{253}{98} \hat{n} \cdot \vec{S}_1 \hat{n} \cdot \vec{v}_2 \vec{S}_1 \cdot \vec{v}_1 + \frac{158}{49} \hat{n} \cdot \vec{S}_1 \hat{n} \cdot \vec{v}_1 \vec{S}_1 \cdot \vec{v}_2 + \\
& 4 \hat{n} \cdot \vec{S}_1 \hat{n} \cdot \vec{v}_2 \vec{S}_1 \cdot \vec{v}_2 - \frac{929 \vec{S}_1 \cdot \vec{v}_1 \vec{S}_1 \cdot \vec{v}_2}{2450} - \frac{1565 \left( \hat{n} \cdot \vec{S}_1 \right)^2 \vec{v}_1 \cdot \vec{v}_1}{2352} + \frac{25129 \vec{S}_1 \cdot \vec{S}_1 \vec{v}_1 \cdot \vec{v}_1}{58800} + \\
& \left. \frac{79}{49} \left( \hat{n} \cdot \vec{S}_1 \right)^2 \vec{v}_1 \cdot \vec{v}_2 - \frac{1357 \vec{S}_1 \cdot \vec{S}_1 \vec{v}_1 \cdot \vec{v}_2}{2450} + \left( \hat{n} \cdot \vec{S}_1 \right)^2 \vec{v}_2 \cdot \vec{v}_2 - \frac{16}{25} \vec{S}_1 \cdot \vec{S}_1 \vec{v}_2 \cdot \vec{v}_2 \right) + \\
& \left( \frac{1}{r^4} \left( \frac{3}{2} \hat{n} \cdot \vec{a}_1 \left( \hat{n} \cdot \vec{S}_1 \right)^2 + \frac{3}{2} \hat{n} \cdot \vec{a}_2 \left( \hat{n} \cdot \vec{S}_1 \right)^2 - \frac{9}{7} \hat{n} \cdot \vec{S}_1 \hat{n} \cdot \vec{v}_1 \hat{n} \cdot \vec{S}_1 - 3 \hat{n} \cdot \vec{S}_1 \hat{n} \cdot \vec{v}_2 \hat{n} \cdot \vec{S}_1 + \right. \right. \\
& \quad \frac{9}{35} \vec{S}_1 \cdot \vec{v}_1 \hat{n} \cdot \vec{S}_1 + \frac{3}{5} \vec{S}_1 \cdot \vec{v}_2 \hat{n} \cdot \vec{S}_1 - \frac{3}{5} \vec{S}_1 \cdot \vec{a}_1 \hat{n} \cdot \vec{S}_1 - \frac{3}{5} \vec{S}_1 \cdot \vec{a}_2 \hat{n} \cdot \vec{S}_1 + \frac{9}{35} \hat{n} \cdot \vec{v}_1 \vec{S}_1 \cdot \vec{S}_1 + \\
& \quad \left. \frac{3}{5} \hat{n} \cdot \vec{v}_2 \vec{S}_1 \cdot \vec{S}_1 - \frac{3}{10} \hat{n} \cdot \vec{a}_1 \vec{S}_1 \cdot \vec{S}_1 - \frac{3}{10} \hat{n} \cdot \vec{a}_2 \vec{S}_1 \cdot \vec{S}_1 + \frac{9}{35} \hat{n} \cdot \vec{S}_1 \vec{S}_1 \cdot \vec{v}_1 + \frac{3}{5} \hat{n} \cdot \vec{S}_1 \vec{S}_1 \cdot \vec{v}_2 \right) + \frac{1}{r^5} \\
& \quad \left( -\frac{9}{4} \left( \hat{n} \cdot \vec{v}_1 \right)^2 \left( \hat{n} \cdot \vec{S}_1 \right)^2 + \frac{21}{2} \left( \hat{n} \cdot \vec{v}_2 \right)^2 \left( \hat{n} \cdot \vec{S}_1 \right)^2 + 12 \hat{n} \cdot \vec{v}_1 \hat{n} \cdot \vec{v}_2 \left( \hat{n} \cdot \vec{S}_1 \right)^2 + \frac{9}{28} \vec{v}_1 \cdot \vec{v}_1 \left( \hat{n} \cdot \vec{S}_1 \right)^2 - \right. \\
& \quad \frac{12}{7} \vec{v}_1 \cdot \vec{v}_2 \left( \hat{n} \cdot \vec{S}_1 \right)^2 - \frac{3}{2} \vec{v}_2 \cdot \vec{v}_2 \left( \hat{n} \cdot \vec{S}_1 \right)^2 + \frac{9}{7} \hat{n} \cdot \vec{v}_1 \vec{S}_1 \cdot \vec{v}_1 \hat{n} \cdot \vec{S}_1 - \frac{24}{7} \hat{n} \cdot \vec{v}_2 \vec{S}_1 \cdot \vec{v}_1 \hat{n} \cdot \vec{S}_1 - \frac{24}{7} \hat{n} \cdot \vec{v}_1 \vec{S}_1 \cdot \vec{v}_2 \\
& \quad \hat{n} \cdot \vec{S}_1 - 6 \hat{n} \cdot \vec{v}_2 \vec{S}_1 \cdot \vec{v}_2 \hat{n} \cdot \vec{S}_1 - \frac{9}{70} \left( \vec{S}_1 \cdot \vec{v}_1 \right)^2 + \frac{3}{5} \left( \vec{S}_1 \cdot \vec{v}_2 \right)^2 + \frac{9}{28} \left( \hat{n} \cdot \vec{v}_1 \right)^2 \vec{S}_1 \cdot \vec{S}_1 - \frac{3}{2} \left( \hat{n} \cdot \vec{v}_2 \right)^2 \vec{S}_1 \cdot \vec{S}_1 - \\
& \quad \left. \frac{12}{7} \hat{n} \cdot \vec{v}_1 \hat{n} \cdot \vec{v}_2 \vec{S}_1 \cdot \vec{S}_1 + \frac{24}{35} \vec{S}_1 \cdot \vec{v}_1 \vec{S}_1 \cdot \vec{v}_2 - \frac{9}{140} \vec{S}_1 \cdot \vec{S}_1 \vec{v}_1 \cdot \vec{v}_1 + \frac{12}{35} \vec{S}_1 \cdot \vec{S}_1 \vec{v}_1 \cdot \vec{v}_2 + \frac{3}{10} \vec{S}_1 \cdot \vec{S}_1 \vec{v}_2 \cdot \vec{v}_2 \right) \Bigg) \\
& \log \left( \frac{r}{R_\theta} \right) + \frac{1}{\epsilon_d} \left( \frac{1}{r^4} \left( -\frac{1}{2} \hat{n} \cdot \vec{a}_1 \left( \hat{n} \cdot \vec{S}_1 \right)^2 - \frac{1}{2} \hat{n} \cdot \vec{a}_2 \left( \hat{n} \cdot \vec{S}_1 \right)^2 + \frac{3}{7} \hat{n} \cdot \vec{S}_1 \hat{n} \cdot \vec{v}_1 \hat{n} \cdot \vec{S}_1 + \hat{n} \cdot \vec{S}_1 \hat{n} \cdot \vec{v}_2 \hat{n} \cdot \vec{S}_1 - \right. \right. \\
& \quad \frac{3}{35} \vec{S}_1 \cdot \vec{v}_1 \hat{n} \cdot \vec{S}_1 - \frac{1}{5} \vec{S}_1 \cdot \vec{v}_2 \hat{n} \cdot \vec{S}_1 + \frac{1}{5} \vec{S}_1 \cdot \vec{a}_1 \hat{n} \cdot \vec{S}_1 + \frac{1}{5} \vec{S}_1 \cdot \vec{a}_2 \hat{n} \cdot \vec{S}_1 - \frac{3}{35} \hat{n} \cdot \vec{v}_1 \vec{S}_1 \cdot \vec{S}_1 - \\
& \quad \left. \frac{1}{5} \hat{n} \cdot \vec{v}_2 \vec{S}_1 \cdot \vec{S}_1 + \frac{1}{10} \hat{n} \cdot \vec{a}_1 \vec{S}_1 \cdot \vec{S}_1 + \frac{1}{10} \hat{n} \cdot \vec{a}_2 \vec{S}_1 \cdot \vec{S}_1 - \frac{3}{35} \hat{n} \cdot \vec{S}_1 \vec{S}_1 \cdot \vec{v}_1 - \frac{1}{5} \hat{n} \cdot \vec{S}_1 \vec{S}_1 \cdot \vec{v}_2 \right) + \frac{1}{r^5} \\
& \quad \left( \frac{3}{4} \left( \hat{n} \cdot \vec{v}_1 \right)^2 \left( \hat{n} \cdot \vec{S}_1 \right)^2 - \frac{7}{2} \left( \hat{n} \cdot \vec{v}_2 \right)^2 \left( \hat{n} \cdot \vec{S}_1 \right)^2 - 4 \hat{n} \cdot \vec{v}_1 \hat{n} \cdot \vec{v}_2 \left( \hat{n} \cdot \vec{S}_1 \right)^2 - \frac{3}{28} \vec{v}_1 \cdot \vec{v}_1 \left( \hat{n} \cdot \vec{S}_1 \right)^2 + \right. \\
& \quad \frac{4}{7} \vec{v}_1 \cdot \vec{v}_2 \left( \hat{n} \cdot \vec{S}_1 \right)^2 + \frac{1}{2} \vec{v}_2 \cdot \vec{v}_2 \left( \hat{n} \cdot \vec{S}_1 \right)^2 - \frac{3}{7} \hat{n} \cdot \vec{v}_1 \vec{S}_1 \cdot \vec{v}_1 \hat{n} \cdot \vec{S}_1 + \frac{8}{7} \hat{n} \cdot \vec{v}_2 \vec{S}_1 \cdot \vec{v}_1 \hat{n} \cdot \vec{S}_1 + \frac{8}{7} \hat{n} \cdot \vec{v}_1 \vec{S}_1 \cdot \vec{v}_2 \hat{n} \cdot \vec{S}_1 + \\
& \quad 2 \hat{n} \cdot \vec{v}_2 \vec{S}_1 \cdot \vec{v}_2 \hat{n} \cdot \vec{S}_1 + \frac{3}{70} \left( \vec{S}_1 \cdot \vec{v}_1 \right)^2 - \frac{1}{5} \left( \vec{S}_1 \cdot \vec{v}_2 \right)^2 - \frac{3}{28} \left( \hat{n} \cdot \vec{v}_1 \right)^2 \vec{S}_1 \cdot \vec{S}_1 + \frac{1}{2} \left( \hat{n} \cdot \vec{v}_2 \right)^2 \vec{S}_1 \cdot \vec{S}_1 + \\
& \quad \left. \left. \frac{4}{7} \hat{n} \cdot \vec{v}_1 \hat{n} \cdot \vec{v}_2 \vec{S}_1 \cdot \vec{S}_1 - \frac{8}{35} \vec{S}_1 \cdot \vec{v}_1 \vec{S}_1 \cdot \vec{v}_2 + \frac{3}{140} \vec{S}_1 \cdot \vec{S}_1 \vec{v}_1 \cdot \vec{v}_1 - \frac{4}{35} \vec{S}_1 \cdot \vec{S}_1 \vec{v}_1 \cdot \vec{v}_2 - \frac{1}{10} \vec{S}_1 \cdot \vec{S}_1 \vec{v}_2 \cdot \vec{v}_2 \right) \right) \Bigg) \Bigg\}
\end{aligned}$$

{DiagS1S1[3, 1, 51],

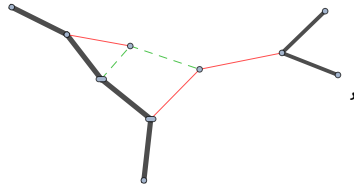

$$G^3 m_1 m_2 \left( \frac{-\frac{2}{5} \vec{S}_1 \cdot \vec{a}_1 \hat{n} \cdot \vec{S}_1 + \frac{2}{5} \vec{S}_1 \cdot \vec{S}_1 \hat{n} \cdot \vec{a}_1 + \frac{2}{5} \vec{S}_1 \cdot \vec{S}_1 \hat{n} \cdot \vec{v}_1 - \frac{2}{5} \hat{n} \cdot \vec{S}_1 \vec{S}_1 \cdot \vec{v}_1}{r^4} + \frac{1}{r^5} \left( \frac{6}{7} \left( \hat{n} \cdot \vec{S}_1 \cdot \vec{v}_1 \right)^2 - \frac{6}{7} \vec{S}_1 \cdot \vec{S}_1 \left( \hat{n} \cdot \vec{v}_1 \right)^2 - \right. \right.$$

$$2 \vec{S}_1 \cdot \vec{S}_1 \hat{n} \cdot \vec{v}_1 \hat{n} \cdot \vec{v}_2 + \frac{6}{7} \hat{n} \cdot \vec{S}_1 \hat{n} \cdot \vec{v}_1 \vec{S}_1 \cdot \vec{v}_1 + 2 \hat{n} \cdot \vec{S}_1 \hat{n} \cdot \vec{v}_2 \vec{S}_1 \cdot \vec{v}_1 - \frac{2}{5} \vec{S}_1 \cdot \vec{v}_1 \vec{S}_1 \cdot \vec{v}_2 + \frac{2}{5} \vec{S}_1 \cdot \vec{S}_1 \vec{v}_1 \cdot \vec{v}_2 \Bigg) \Bigg\}$$

{DiagS1S1 [3, 1, 52], 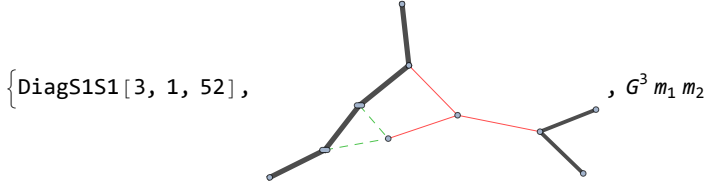 ,  $G^3 m_1 m_2$

$$\left( \frac{\frac{16}{49} \hat{n} \cdot \vec{S}_1 \hat{n} \cdot \vec{S}_1 \hat{n} \cdot \vec{v}_1 + \frac{4 \vec{S}_1 \cdot \vec{S}_1 \hat{n} \cdot \vec{v}_1}{1225} + \frac{144 \hat{n} \cdot \vec{S}_1 \vec{S}_1 \cdot \vec{v}_1}{1225} - \frac{12}{25} \hat{n} \cdot \vec{S}_1 \vec{S}_1 \cdot \vec{v}_2 - \frac{12}{25} \hat{n} \cdot \vec{v}_2 \vec{S}_1 \cdot \vec{S}_1 + \frac{144 \hat{n} \cdot \vec{S}_1 \vec{S}_1 \cdot \vec{v}_1}{1225} - \frac{12}{25} \hat{n} \cdot \vec{S}_1 \vec{S}_1 \cdot \vec{v}_2}{r^4} + \right. \\ \left. \frac{1}{r^5} \left( -\frac{4}{3} (\hat{n} \cdot \vec{v}_1)^2 (\hat{n} \cdot \vec{S}_1)^2 + 6 \hat{n} \cdot \vec{v}_1 \hat{n} \cdot \vec{v}_2 (\hat{n} \cdot \vec{S}_1)^2 - \frac{4}{49} \vec{v}_1 \cdot \vec{v}_1 (\hat{n} \cdot \vec{S}_1)^2 + \frac{12}{49} \hat{n} \cdot \vec{v}_1 \vec{S}_1 \cdot \vec{v}_1 \hat{n} \cdot \vec{S}_1 + \right. \right. \\ \left. \left. \frac{218 (\vec{S}_1 \cdot \vec{v}_1)^2}{3675} + \frac{16}{147} (\hat{n} \cdot \vec{v}_1)^2 \vec{S}_1 \cdot \vec{S}_1 - \frac{12}{25} \vec{S}_1 \cdot \vec{v}_1 \vec{S}_1 \cdot \vec{v}_2 + \frac{74 \vec{S}_1 \cdot \vec{S}_1 \vec{v}_1 \cdot \vec{v}_1}{3675} - \frac{6}{25} \vec{S}_1 \cdot \vec{S}_1 \vec{v}_1 \cdot \vec{v}_2 \right) + \right. \\ \left( \frac{1}{r^4} \left( -\frac{12}{7} \hat{n} \cdot \vec{S}_1 \hat{n} \cdot \vec{S}_1 \hat{n} \cdot \vec{v}_1 + \frac{12}{35} \vec{S}_1 \cdot \vec{S}_1 \hat{n} \cdot \vec{v}_1 + 12 \hat{n} \cdot \vec{S}_1 \hat{n} \cdot \vec{S}_1 \hat{n} \cdot \vec{v}_2 + \frac{12}{35} \hat{n} \cdot \vec{S}_1 \vec{S}_1 \cdot \vec{v}_1 - \right. \right. \\ \left. \left. \frac{12}{5} \hat{n} \cdot \vec{S}_1 \vec{S}_1 \cdot \vec{v}_2 - \frac{12}{5} \hat{n} \cdot \vec{v}_2 \vec{S}_1 \cdot \vec{S}_1 + \frac{12}{35} \hat{n} \cdot \vec{S}_1 \vec{S}_1 \cdot \vec{v}_1 - \frac{12}{5} \hat{n} \cdot \vec{S}_1 \vec{S}_1 \cdot \vec{v}_2 \right) + \frac{1}{r^5} \right. \\ \left( 4 (\hat{n} \cdot \vec{v}_1)^2 (\hat{n} \cdot \vec{S}_1)^2 - 42 \hat{n} \cdot \vec{v}_1 \hat{n} \cdot \vec{v}_2 (\hat{n} \cdot \vec{S}_1)^2 - \frac{4}{7} \vec{v}_1 \cdot \vec{v}_1 (\hat{n} \cdot \vec{S}_1)^2 + 6 \vec{v}_1 \cdot \vec{v}_2 (\hat{n} \cdot \vec{S}_1)^2 - \right. \\ \left. \frac{16}{7} \hat{n} \cdot \vec{v}_1 \vec{S}_1 \cdot \vec{v}_1 \hat{n} \cdot \vec{S}_1 + 12 \hat{n} \cdot \vec{v}_2 \vec{S}_1 \cdot \vec{v}_1 \hat{n} \cdot \vec{S}_1 + 12 \hat{n} \cdot \vec{v}_1 \vec{S}_1 \cdot \vec{v}_2 \hat{n} \cdot \vec{S}_1 + \frac{8}{35} (\vec{S}_1 \cdot \vec{v}_1)^2 - \frac{4}{7} (\hat{n} \cdot \vec{v}_1)^2 \vec{S}_1 \cdot \vec{S}_1 + \right. \\ \left. \left. 6 \hat{n} \cdot \vec{v}_1 \hat{n} \cdot \vec{v}_2 \vec{S}_1 \cdot \vec{S}_1 - \frac{12}{5} \vec{S}_1 \cdot \vec{v}_1 \vec{S}_1 \cdot \vec{v}_2 + \frac{4}{35} \vec{S}_1 \cdot \vec{S}_1 \vec{v}_1 \cdot \vec{v}_1 - \frac{6}{5} \vec{S}_1 \cdot \vec{S}_1 \vec{v}_1 \cdot \vec{v}_2 \right) \right) \log \left( \frac{r}{R_0} \right) + \\ \frac{1}{\epsilon_d} \left( \frac{1}{r^4} \left( \frac{4}{7} \hat{n} \cdot \vec{S}_1 \hat{n} \cdot \vec{S}_1 \hat{n} \cdot \vec{v}_1 - \frac{4}{35} \vec{S}_1 \cdot \vec{S}_1 \hat{n} \cdot \vec{v}_1 - 4 \hat{n} \cdot \vec{S}_1 \hat{n} \cdot \vec{S}_1 \hat{n} \cdot \vec{v}_2 - \frac{4}{35} \hat{n} \cdot \vec{S}_1 \vec{S}_1 \cdot \vec{v}_1 + \right. \right. \\ \left. \left. \frac{4}{5} \hat{n} \cdot \vec{S}_1 \vec{S}_1 \cdot \vec{v}_2 + \frac{4}{5} \hat{n} \cdot \vec{v}_2 \vec{S}_1 \cdot \vec{S}_1 - \frac{4}{35} \hat{n} \cdot \vec{S}_1 \vec{S}_1 \cdot \vec{v}_1 + \frac{4}{5} \hat{n} \cdot \vec{S}_1 \vec{S}_1 \cdot \vec{v}_2 \right) + \frac{1}{r^5} \right. \\ \left( -\frac{4}{3} (\hat{n} \cdot \vec{v}_1)^2 (\hat{n} \cdot \vec{S}_1)^2 + 14 \hat{n} \cdot \vec{v}_1 \hat{n} \cdot \vec{v}_2 (\hat{n} \cdot \vec{S}_1)^2 + \frac{4}{21} \vec{v}_1 \cdot \vec{v}_1 (\hat{n} \cdot \vec{S}_1)^2 - 2 \vec{v}_1 \cdot \vec{v}_2 (\hat{n} \cdot \vec{S}_1)^2 + \right. \\ \left. \frac{16}{21} \hat{n} \cdot \vec{v}_1 \vec{S}_1 \cdot \vec{v}_1 \hat{n} \cdot \vec{S}_1 - 4 \hat{n} \cdot \vec{v}_2 \vec{S}_1 \cdot \vec{v}_1 \hat{n} \cdot \vec{S}_1 - 4 \hat{n} \cdot \vec{v}_1 \vec{S}_1 \cdot \vec{v}_2 \hat{n} \cdot \vec{S}_1 - \frac{8}{105} (\vec{S}_1 \cdot \vec{v}_1)^2 + \right. \\ \left. \left. \frac{4}{21} (\hat{n} \cdot \vec{v}_1)^2 \vec{S}_1 \cdot \vec{S}_1 - 2 \hat{n} \cdot \vec{v}_1 \hat{n} \cdot \vec{v}_2 \vec{S}_1 \cdot \vec{S}_1 + \frac{4}{5} \vec{S}_1 \cdot \vec{v}_1 \vec{S}_1 \cdot \vec{v}_2 - \frac{4}{105} \vec{S}_1 \cdot \vec{S}_1 \vec{v}_1 \cdot \vec{v}_1 + \frac{2}{5} \vec{S}_1 \cdot \vec{S}_1 \vec{v}_1 \cdot \vec{v}_2 \right) \right) \Bigg\}$$

{DiagS1S1 [3, 1, 53], 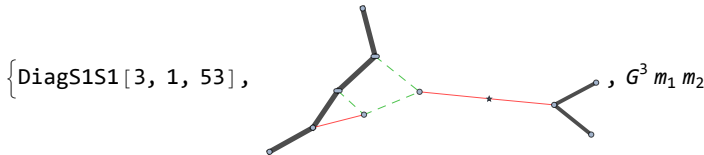 ,  $G^3 m_1 m_2$

$$\left( \frac{\frac{26}{49} \hat{n} \cdot \vec{S}_1 \hat{n} \cdot \vec{S}_1 \hat{n} \cdot \vec{v}_2 - \frac{634 \vec{S}_1 \cdot \vec{S}_1 \hat{n} \cdot \vec{v}_2}{1225} - \frac{214 \hat{n} \cdot \vec{S}_1 \vec{S}_1 \cdot \vec{v}_2}{1225} - \frac{214 \hat{n} \cdot \vec{S}_1 \vec{S}_1 \cdot \vec{v}_2}{1225}}{r^4} + \frac{1}{r^5} \left( -(\hat{n} \cdot \vec{v}_1) \hat{n} \cdot \vec{v}_2 (\hat{n} \cdot \vec{S}_1)^2 + \frac{13}{49} \vec{v}_1 \cdot \vec{v}_2 (\hat{n} \cdot \vec{S}_1)^2 + \right. \right.$$

$$\begin{aligned}
& \frac{26}{49} \hat{n} \cdot \vec{v}_2 \vec{S}_1 \cdot \vec{v}_1 \hat{n} \cdot \vec{S}_1 + \frac{26}{49} \hat{n} \cdot \vec{v}_1 \vec{S}_1 \cdot \vec{v}_2 \hat{n} \cdot \vec{S}_1 + \frac{55}{49} \hat{n} \cdot \vec{v}_1 \hat{n} \cdot \vec{v}_2 \vec{S}_1 \cdot \vec{S}_1 - \frac{214 \vec{S}_1 \cdot \vec{v}_1 \vec{S}_1 \cdot \vec{v}_2}{1225} - \frac{317 \vec{S}_1 \cdot \vec{S}_1 \vec{v}_1 \cdot \vec{v}_2}{1225} \Bigg) + \\
& \left( \frac{\frac{12}{7} \hat{n} \cdot \vec{S}_1 \hat{n} \cdot \vec{S}_1 \hat{n} \cdot \vec{v}_2 - \frac{12}{35} \vec{S}_1 \cdot \vec{S}_1 \hat{n} \cdot \vec{v}_2 - \frac{12}{35} \hat{n} \cdot \vec{S}_1 \vec{S}_1 \cdot \vec{v}_2 - \frac{12}{35} \hat{n} \cdot \vec{S}_1 \vec{S}_1 \cdot \vec{v}_2}{r^4} + \frac{1}{r^5} \right. \\
& \quad \left( -6 \hat{n} \cdot \vec{v}_1 \hat{n} \cdot \vec{v}_2 (\hat{n} \cdot \vec{S}_1)^2 + \frac{6}{7} \vec{v}_1 \cdot \vec{v}_2 (\hat{n} \cdot \vec{S}_1)^2 + \frac{12}{7} \hat{n} \cdot \vec{v}_2 \vec{S}_1 \cdot \vec{v}_1 \hat{n} \cdot \vec{S}_1 + \frac{12}{7} \hat{n} \cdot \vec{v}_1 \vec{S}_1 \cdot \vec{v}_2 \hat{n} \cdot \vec{S}_1 + \right. \\
& \quad \left. \frac{6}{7} \hat{n} \cdot \vec{v}_1 \hat{n} \cdot \vec{v}_2 \vec{S}_1 \cdot \vec{S}_1 - \frac{12}{35} \vec{S}_1 \cdot \vec{v}_1 \vec{S}_1 \cdot \vec{v}_2 - \frac{6}{35} \vec{S}_1 \cdot \vec{S}_1 \vec{v}_1 \cdot \vec{v}_2 \right) \log\left(\frac{r}{R_\theta}\right) + \\
& \quad \left. \frac{1}{\epsilon_d} \left( \frac{-\frac{4}{7} \hat{n} \cdot \vec{S}_1 \hat{n} \cdot \vec{S}_1 \hat{n} \cdot \vec{v}_2 + \frac{4}{35} \vec{S}_1 \cdot \vec{S}_1 \hat{n} \cdot \vec{v}_2 + \frac{4}{35} \hat{n} \cdot \vec{S}_1 \vec{S}_1 \cdot \vec{v}_2 + \frac{4}{35} \hat{n} \cdot \vec{S}_1 \vec{S}_1 \cdot \vec{v}_2}{r^4} + \frac{1}{r^5} \right. \right. \\
& \quad \left( 2 \hat{n} \cdot \vec{v}_1 \hat{n} \cdot \vec{v}_2 (\hat{n} \cdot \vec{S}_1)^2 - \frac{2}{7} \vec{v}_1 \cdot \vec{v}_2 (\hat{n} \cdot \vec{S}_1)^2 - \frac{4}{7} \hat{n} \cdot \vec{v}_2 \vec{S}_1 \cdot \vec{v}_1 \hat{n} \cdot \vec{S}_1 - \right. \\
& \quad \left. \frac{4}{7} \hat{n} \cdot \vec{v}_1 \vec{S}_1 \cdot \vec{v}_2 \hat{n} \cdot \vec{S}_1 - \frac{2}{7} \hat{n} \cdot \vec{v}_1 \hat{n} \cdot \vec{v}_2 \vec{S}_1 \cdot \vec{S}_1 + \frac{4}{35} \vec{S}_1 \cdot \vec{v}_1 \vec{S}_1 \cdot \vec{v}_2 + \frac{2}{35} \vec{S}_1 \cdot \vec{S}_1 \vec{v}_1 \cdot \vec{v}_2 \right) \Bigg) \Bigg\}
\end{aligned}$$

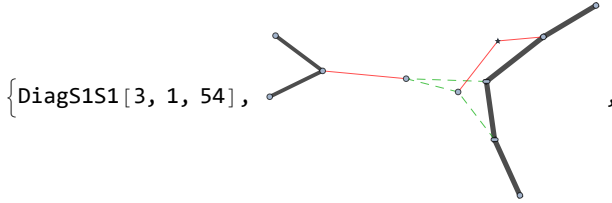

$$\begin{aligned}
& G^3 m_1 m_2 \left( \frac{-\frac{136}{49} \hat{n} \cdot \vec{S}_1 \hat{n} \cdot \vec{S}_1 \hat{n} \cdot \vec{v}_1 - \frac{242}{245} \vec{S}_1 \cdot \vec{S}_1 \hat{n} \cdot \vec{v}_1 + \frac{157}{245} \hat{n} \cdot \vec{S}_1 \vec{S}_1 \cdot \vec{v}_1 + \frac{157}{245} \hat{n} \cdot \vec{S}_1 \vec{S}_1 \cdot \vec{v}_1}{r^4} + \frac{1}{r^5} \right. \\
& \quad \left( \frac{2}{7} (\hat{n} \times \vec{S}_1 \cdot \vec{v}_1)^2 + \frac{34}{3} (\hat{n} \cdot \vec{S}_1)^2 (\hat{n} \cdot \vec{v}_1)^2 + \frac{3763 (\vec{S}_1 \cdot \vec{v}_1)^2}{3675} - 14 (\hat{n} \cdot \vec{S}_1)^2 \hat{n} \cdot \vec{v}_1 \hat{n} \cdot \vec{v}_2 + \frac{239}{147} (\hat{n} \cdot \vec{v}_1)^2 \vec{S}_1 \cdot \vec{S}_1 - \right. \\
& \quad \frac{79}{49} \hat{n} \cdot \vec{v}_1 \hat{n} \cdot \vec{v}_2 \vec{S}_1 \cdot \vec{S}_1 - \frac{941}{147} \hat{n} \cdot \vec{S}_1 \hat{n} \cdot \vec{v}_1 \vec{S}_1 \cdot \vec{v}_1 + \frac{241}{49} \hat{n} \cdot \vec{S}_1 \hat{n} \cdot \vec{v}_2 \vec{S}_1 \cdot \vec{v}_1 + \frac{136}{49} \hat{n} \cdot \vec{S}_1 \hat{n} \cdot \vec{v}_1 \vec{S}_1 \cdot \vec{v}_2 - \\
& \quad \frac{157}{245} \vec{S}_1 \cdot \vec{v}_1 \vec{S}_1 \cdot \vec{v}_2 - \frac{104}{147} (\hat{n} \cdot \vec{S}_1)^2 \vec{v}_1 \cdot \vec{v}_1 - \frac{697 \vec{S}_1 \cdot \vec{S}_1 \vec{v}_1 \cdot \vec{v}_1}{1225} + \frac{68}{49} (\hat{n} \cdot \vec{S}_1)^2 \vec{v}_1 \cdot \vec{v}_2 + \frac{121}{245} \vec{S}_1 \cdot \vec{S}_1 \vec{v}_1 \cdot \vec{v}_2 \Bigg) + \\
& \quad \left( \frac{\frac{60}{7} \hat{n} \cdot \vec{S}_1 \hat{n} \cdot \vec{S}_1 \hat{n} \cdot \vec{v}_1 - \frac{12}{7} \vec{S}_1 \cdot \vec{S}_1 \hat{n} \cdot \vec{v}_1 - \frac{12}{7} \hat{n} \cdot \vec{S}_1 \vec{S}_1 \cdot \vec{v}_1 - \frac{12}{7} \hat{n} \cdot \vec{S}_1 \vec{S}_1 \cdot \vec{v}_1}{r^4} + \frac{1}{r^5} \right. \\
& \quad \left( -26 (\hat{n} \cdot \vec{v}_1)^2 (\hat{n} \cdot \vec{S}_1)^2 + 30 \hat{n} \cdot \vec{v}_1 \hat{n} \cdot \vec{v}_2 (\hat{n} \cdot \vec{S}_1)^2 + \frac{26}{7} \vec{v}_1 \cdot \vec{v}_1 (\hat{n} \cdot \vec{S}_1)^2 - \frac{30}{7} \vec{v}_1 \cdot \vec{v}_2 (\hat{n} \cdot \vec{S}_1)^2 + \right. \\
& \quad \frac{104}{7} \hat{n} \cdot \vec{v}_1 \vec{S}_1 \cdot \vec{v}_1 \hat{n} \cdot \vec{S}_1 - \frac{60}{7} \hat{n} \cdot \vec{v}_2 \vec{S}_1 \cdot \vec{v}_1 \hat{n} \cdot \vec{S}_1 - \frac{60}{7} \hat{n} \cdot \vec{v}_1 \vec{S}_1 \cdot \vec{v}_2 \hat{n} \cdot \vec{S}_1 - \frac{52}{35} (\vec{S}_1 \cdot \vec{v}_1)^2 + \\
& \quad \left. \frac{26}{7} (\hat{n} \cdot \vec{v}_1)^2 \vec{S}_1 \cdot \vec{S}_1 - \frac{30}{7} \hat{n} \cdot \vec{v}_1 \hat{n} \cdot \vec{v}_2 \vec{S}_1 \cdot \vec{S}_1 + \frac{12}{7} \vec{S}_1 \cdot \vec{v}_1 \vec{S}_1 \cdot \vec{v}_2 - \frac{26}{35} \vec{S}_1 \cdot \vec{S}_1 \vec{v}_1 \cdot \vec{v}_1 + \frac{6}{7} \vec{S}_1 \cdot \vec{S}_1 \vec{v}_1 \cdot \vec{v}_2 \right) \Bigg)
\end{aligned}$$

$$\log\left(\frac{r}{R_\theta}\right) + \frac{1}{\epsilon_d} \left( \frac{-\frac{20}{7} \hat{n} \cdot \vec{S}_1 \hat{n} \cdot \vec{S}_1 \hat{n} \cdot \vec{v}_1 + \frac{4}{7} \vec{S}_1 \cdot \vec{S}_1 \hat{n} \cdot \vec{v}_1 + \frac{4}{7} \hat{n} \cdot \vec{S}_1 \vec{S}_1 \cdot \vec{v}_1 + \frac{4}{7} \hat{n} \cdot \vec{S}_1 \vec{S}_1 \cdot \vec{v}_1}{r^4} + \frac{1}{r^5} \right. \\ \left. \left( \frac{26}{3} (\hat{n} \cdot \vec{v}_1)^2 (\hat{n} \cdot \vec{S}_1)^2 - 10 \hat{n} \cdot \vec{v}_1 \hat{n} \cdot \vec{v}_2 (\hat{n} \cdot \vec{S}_1)^2 - \frac{26}{21} \vec{v}_1 \cdot \vec{v}_1 (\hat{n} \cdot \vec{S}_1)^2 + \frac{10}{7} \vec{v}_1 \cdot \vec{v}_2 (\hat{n} \cdot \vec{S}_1)^2 - \right. \right. \\ \left. \frac{104}{21} \hat{n} \cdot \vec{v}_1 \vec{S}_1 \cdot \vec{v}_1 \hat{n} \cdot \vec{S}_1 + \frac{20}{7} \hat{n} \cdot \vec{v}_2 \vec{S}_1 \cdot \vec{v}_1 \hat{n} \cdot \vec{S}_1 + \frac{20}{7} \hat{n} \cdot \vec{v}_1 \vec{S}_1 \cdot \vec{v}_2 \hat{n} \cdot \vec{S}_1 + \frac{52}{105} (\vec{S}_1 \cdot \vec{v}_1)^2 - \right. \\ \left. \left. \frac{26}{21} (\hat{n} \cdot \vec{v}_1)^2 \vec{S}_1 \cdot \vec{S}_1 + \frac{10}{7} \hat{n} \cdot \vec{v}_1 \hat{n} \cdot \vec{v}_2 \vec{S}_1 \cdot \vec{S}_1 - \frac{4}{7} \vec{S}_1 \cdot \vec{v}_1 \vec{S}_1 \cdot \vec{v}_2 + \frac{26}{105} \vec{S}_1 \cdot \vec{S}_1 \vec{v}_1 \cdot \vec{v}_1 - \frac{2}{7} \vec{S}_1 \cdot \vec{S}_1 \vec{v}_1 \cdot \vec{v}_2 \right) \right) \Bigg\}$$

{DiagS1S1[3, 1, 55],

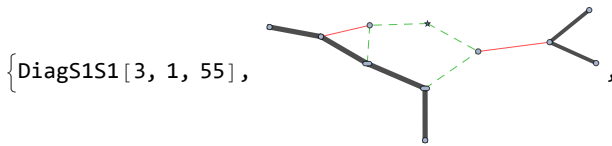

$$G^3 m_1 m_2 \left( \frac{\left( \frac{28}{25} (\hat{n} \cdot \vec{S}_1)^2 - \frac{8}{75} \vec{S}_1 \cdot \vec{S}_1 \right)}{r^3} + \frac{1}{r^4} \left( -8 \hat{n} \cdot \vec{S}_1 \hat{n} \cdot \vec{S}_1 \hat{n} \cdot \vec{v}_1 + \frac{28}{25} \vec{S}_1 \cdot \vec{S}_1 \hat{n} \cdot \vec{v}_1 + 8 \hat{n} \cdot \vec{S}_1 \hat{n} \cdot \vec{S}_1 \hat{n} \cdot \vec{v}_2 - \right. \right. \\ \left. \frac{2}{25} \hat{n} \cdot \vec{S}_1 \vec{S}_1 \cdot \vec{v}_1 - \frac{28}{25} \hat{n} \cdot \vec{S}_1 \vec{S}_1 \cdot \vec{v}_2 - \frac{28}{25} \hat{n} \cdot \vec{v}_2 \vec{S}_1 \cdot \vec{S}_1 + \frac{58}{25} \hat{n} \cdot \vec{S}_1 \vec{S}_1 \cdot \vec{v}_1 - \frac{28}{25} \hat{n} \cdot \vec{S}_1 \vec{S}_1 \cdot \vec{v}_2 \right) + \frac{1}{r^5} \\ \left( -\frac{12}{7} (\hat{n} \cdot \vec{S}_1 \cdot \vec{v}_1)^2 + 13 (\hat{n} \cdot \vec{S}_1)^2 (\hat{n} \cdot \vec{v}_1)^2 - \frac{108}{175} (\vec{S}_1 \cdot \vec{v}_1)^2 - 29 (\hat{n} \cdot \vec{S}_1)^2 \hat{n} \cdot \vec{v}_1 \hat{n} \cdot \vec{v}_2 - \frac{23}{7} (\hat{n} \cdot \vec{v}_1)^2 \vec{S}_1 \cdot \vec{S}_1 + \right. \\ \frac{173}{49} \hat{n} \cdot \vec{v}_1 \hat{n} \cdot \vec{v}_2 \vec{S}_1 \cdot \vec{S}_1 - \frac{94}{21} \hat{n} \cdot \vec{S}_1 \hat{n} \cdot \vec{v}_1 \vec{S}_1 \cdot \vec{v}_1 + \frac{304}{49} \hat{n} \cdot \vec{S}_1 \hat{n} \cdot \vec{v}_2 \vec{S}_1 \cdot \vec{v}_1 + \frac{346}{49} \hat{n} \cdot \vec{S}_1 \hat{n} \cdot \vec{v}_1 \vec{S}_1 \cdot \vec{v}_2 - \\ \frac{44}{49} \vec{S}_1 \cdot \vec{v}_1 \vec{S}_1 \cdot \vec{v}_2 - \frac{37}{21} (\hat{n} \cdot \vec{S}_1)^2 \vec{v}_1 \cdot \vec{v}_1 + \frac{943}{525} \vec{S}_1 \cdot \vec{S}_1 \vec{v}_1 \cdot \vec{v}_1 + \frac{173}{49} (\hat{n} \cdot \vec{S}_1)^2 \vec{v}_1 \cdot \vec{v}_2 - \frac{131}{245} \vec{S}_1 \cdot \vec{S}_1 \vec{v}_1 \cdot \vec{v}_2 \Bigg) + \\ \left( \frac{\frac{4}{5} \vec{S}_1 \cdot \vec{S}_1 - \frac{12}{5} (\hat{n} \cdot \vec{S}_1)^2}{r^3} + \frac{1}{r^4} \left( 12 \hat{n} \cdot \vec{S}_1 \hat{n} \cdot \vec{S}_1 \hat{n} \cdot \vec{v}_1 - \frac{12}{5} \vec{S}_1 \cdot \vec{S}_1 \hat{n} \cdot \vec{v}_1 - 12 \hat{n} \cdot \vec{S}_1 \hat{n} \cdot \vec{S}_1 \hat{n} \cdot \vec{v}_2 - \right. \right. \\ \frac{12}{5} \hat{n} \cdot \vec{S}_1 \vec{S}_1 \cdot \vec{v}_1 + \frac{12}{5} \hat{n} \cdot \vec{S}_1 \vec{S}_1 \cdot \vec{v}_2 + \frac{12}{5} \hat{n} \cdot \vec{v}_2 \vec{S}_1 \cdot \vec{S}_1 - \frac{12}{5} \hat{n} \cdot \vec{S}_1 \vec{S}_1 \cdot \vec{v}_1 + \frac{12}{5} \hat{n} \cdot \vec{S}_1 \vec{S}_1 \cdot \vec{v}_2 \Bigg) + \\ \frac{1}{r^5} \left( -14 (\hat{n} \cdot \vec{v}_1)^2 (\hat{n} \cdot \vec{S}_1)^2 + 30 \hat{n} \cdot \vec{v}_1 \hat{n} \cdot \vec{v}_2 (\hat{n} \cdot \vec{S}_1)^2 + 2 \vec{v}_1 \cdot \vec{v}_1 (\hat{n} \cdot \vec{S}_1)^2 - \frac{30}{7} \vec{v}_1 \cdot \vec{v}_2 (\hat{n} \cdot \vec{S}_1)^2 + \right. \\ \left. 8 \hat{n} \cdot \vec{v}_1 \vec{S}_1 \cdot \vec{v}_1 \hat{n} \cdot \vec{S}_1 - \frac{60}{7} \hat{n} \cdot \vec{v}_2 \vec{S}_1 \cdot \vec{v}_1 \hat{n} \cdot \vec{S}_1 - \frac{60}{7} \hat{n} \cdot \vec{v}_1 \vec{S}_1 \cdot \vec{v}_2 \hat{n} \cdot \vec{S}_1 - \frac{4}{5} (\vec{S}_1 \cdot \vec{v}_1)^2 + 2 (\hat{n} \cdot \vec{v}_1)^2 \vec{S}_1 \cdot \vec{S}_1 - \right. \\ \left. \frac{30}{7} \hat{n} \cdot \vec{v}_1 \hat{n} \cdot \vec{v}_2 \vec{S}_1 \cdot \vec{S}_1 + \frac{12}{7} \vec{S}_1 \cdot \vec{v}_1 \vec{S}_1 \cdot \vec{v}_2 - \frac{2}{5} \vec{S}_1 \cdot \vec{S}_1 \vec{v}_1 \cdot \vec{v}_1 + \frac{6}{7} \vec{S}_1 \cdot \vec{S}_1 \vec{v}_1 \cdot \vec{v}_2 \right) \Bigg) \log\left(\frac{r}{R_\theta}\right) + \\ \frac{1}{\epsilon_d} \left( \frac{\left( \frac{4}{5} (\hat{n} \cdot \vec{S}_1)^2 - \frac{4}{15} \vec{S}_1 \cdot \vec{S}_1 \right)}{r^3} + \frac{1}{r^4} \left( -4 \hat{n} \cdot \vec{S}_1 \hat{n} \cdot \vec{S}_1 \hat{n} \cdot \vec{v}_1 + \frac{4}{5} \vec{S}_1 \cdot \vec{S}_1 \hat{n} \cdot \vec{v}_1 + 4 \hat{n} \cdot \vec{S}_1 \hat{n} \cdot \vec{S}_1 \hat{n} \cdot \vec{v}_2 + \right. \right. \\ \left. \frac{4}{5} \hat{n} \cdot \vec{S}_1 \vec{S}_1 \cdot \vec{v}_1 - \frac{4}{5} \hat{n} \cdot \vec{S}_1 \vec{S}_1 \cdot \vec{v}_2 - \frac{4}{5} \hat{n} \cdot \vec{v}_2 \vec{S}_1 \cdot \vec{S}_1 + \frac{4}{5} \hat{n} \cdot \vec{S}_1 \vec{S}_1 \cdot \vec{v}_1 - \frac{4}{5} \hat{n} \cdot \vec{S}_1 \vec{S}_1 \cdot \vec{v}_2 \right) + \frac{1}{r^5}$$

$$\left( \frac{14}{3} (\hat{n} \cdot \vec{v}_1)^2 (\hat{n} \cdot \vec{S}_1)^2 - 10 \hat{n} \cdot \vec{v}_1 \hat{n} \cdot \vec{v}_2 (\hat{n} \cdot \vec{S}_1)^2 - \frac{2}{3} \vec{v}_1 \cdot \vec{v}_1 (\hat{n} \cdot \vec{S}_1)^2 + \frac{10}{7} \vec{v}_1 \cdot \vec{v}_2 (\hat{n} \cdot \vec{S}_1)^2 - \right. \\ \left. \frac{8}{3} \hat{n} \cdot \vec{v}_1 \vec{S}_1 \cdot \vec{v}_1 \hat{n} \cdot \vec{S}_1 + \frac{20}{7} \hat{n} \cdot \vec{v}_2 \vec{S}_1 \cdot \vec{v}_1 \hat{n} \cdot \vec{S}_1 + \frac{20}{7} \hat{n} \cdot \vec{v}_1 \vec{S}_1 \cdot \vec{v}_2 \hat{n} \cdot \vec{S}_1 + \frac{4}{15} (\vec{S}_1 \cdot \vec{v}_1)^2 - \right. \\ \left. \frac{2}{3} (\hat{n} \cdot \vec{v}_1)^2 \vec{S}_1 \cdot \vec{S}_1 + \frac{10}{7} \hat{n} \cdot \vec{v}_1 \hat{n} \cdot \vec{v}_2 \vec{S}_1 \cdot \vec{S}_1 - \frac{4}{7} \vec{S}_1 \cdot \vec{v}_1 \vec{S}_1 \cdot \vec{v}_2 + \frac{2}{15} \vec{S}_1 \cdot \vec{S}_1 \vec{v}_1 \cdot \vec{v}_1 - \frac{2}{7} \vec{S}_1 \cdot \vec{S}_1 \vec{v}_1 \cdot \vec{v}_2 \right) \Bigg\}$$

{DiagS1S1[3, 1, 56],

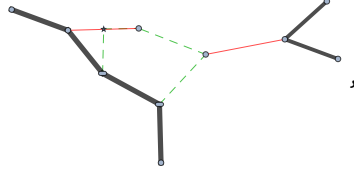

$$G^3 m_1 m_2 \left( \frac{\frac{68}{25} (\hat{n} \cdot \vec{S}_1)^2 + \frac{52}{75} \vec{S}_1 \cdot \vec{S}_1}{r^3} + \frac{1}{r^4} \left( -28 \hat{n} \cdot \vec{S}_1 \hat{n} \cdot \vec{S}_1 \hat{n} \cdot \vec{v}_1 + \frac{68}{25} \vec{S}_1 \cdot \vec{S}_1 \hat{n} \cdot \vec{v}_1 + 28 \hat{n} \cdot \vec{S}_1 \hat{n} \cdot \vec{S}_1 \hat{n} \cdot \vec{v}_2 - \right. \right. \\ \left. \frac{27}{25} \hat{n} \cdot \vec{S}_1 \vec{S}_1 \cdot \vec{v}_1 - \frac{68}{25} \hat{n} \cdot \vec{S}_1 \vec{S}_1 \cdot \vec{v}_2 - \frac{68}{25} \hat{n} \cdot \vec{v}_2 \vec{S}_1 \cdot \vec{S}_1 + \frac{163}{25} \hat{n} \cdot \vec{S}_1 \vec{S}_1 \cdot \vec{v}_1 - \frac{68}{25} \hat{n} \cdot \vec{S}_1 \vec{S}_1 \cdot \vec{v}_2 \right) + \frac{1}{r^5} \\ \left( -4 (\hat{n} \cdot \vec{S}_1 \cdot \vec{v}_1)^2 + 38 (\hat{n} \cdot \vec{S}_1)^2 (\hat{n} \cdot \vec{v}_1)^2 - \frac{1751 (\vec{S}_1 \cdot \vec{v}_1)^2}{1225} - 62 (\hat{n} \cdot \vec{S}_1)^2 \hat{n} \cdot \vec{v}_1 \hat{n} \cdot \vec{v}_2 - \frac{429}{49} (\hat{n} \cdot \vec{v}_1)^2 \vec{S}_1 \cdot \vec{S}_1 + \right. \\ \left. \frac{393}{49} \hat{n} \cdot \vec{v}_1 \hat{n} \cdot \vec{v}_2 \vec{S}_1 \cdot \vec{S}_1 - \frac{589}{49} \hat{n} \cdot \vec{S}_1 \hat{n} \cdot \vec{v}_1 \vec{S}_1 \cdot \vec{v}_1 + \frac{513}{49} \hat{n} \cdot \vec{S}_1 \hat{n} \cdot \vec{v}_2 \vec{S}_1 \cdot \vec{v}_1 + \frac{688}{49} \hat{n} \cdot \vec{S}_1 \hat{n} \cdot \vec{v}_1 \vec{S}_1 \cdot \vec{v}_2 - \right. \\ \left. \frac{261}{245} \vec{S}_1 \cdot \vec{v}_1 \vec{S}_1 \cdot \vec{v}_2 - \frac{240}{49} (\hat{n} \cdot \vec{S}_1)^2 \vec{v}_1 \cdot \vec{v}_1 + \frac{4847 \vec{S}_1 \cdot \vec{S}_1 \vec{v}_1 \cdot \vec{v}_1}{1225} + \frac{344}{49} (\hat{n} \cdot \vec{S}_1)^2 \vec{v}_1 \cdot \vec{v}_2 - \frac{267}{245} \vec{S}_1 \cdot \vec{S}_1 \vec{v}_1 \cdot \vec{v}_2 \right) + \\ \left( \frac{\frac{24}{5} \vec{S}_1 \cdot \vec{S}_1 - \frac{72}{5} (\hat{n} \cdot \vec{S}_1)^2}{r^3} + \frac{1}{r^4} \left( 72 \hat{n} \cdot \vec{S}_1 \hat{n} \cdot \vec{S}_1 \hat{n} \cdot \vec{v}_1 - \frac{72}{5} \vec{S}_1 \cdot \vec{S}_1 \hat{n} \cdot \vec{v}_1 - 72 \hat{n} \cdot \vec{S}_1 \hat{n} \cdot \vec{S}_1 \hat{n} \cdot \vec{v}_2 - \right. \right. \\ \left. \frac{72}{5} \hat{n} \cdot \vec{S}_1 \vec{S}_1 \cdot \vec{v}_1 + \frac{72}{5} \hat{n} \cdot \vec{S}_1 \vec{S}_1 \cdot \vec{v}_2 + \frac{72}{5} \hat{n} \cdot \vec{v}_2 \vec{S}_1 \cdot \vec{S}_1 - \frac{72}{5} \hat{n} \cdot \vec{S}_1 \vec{S}_1 \cdot \vec{v}_1 + \frac{72}{5} \hat{n} \cdot \vec{S}_1 \vec{S}_1 \cdot \vec{v}_2 \right) + \frac{1}{r^5} \\ \left( -54 (\hat{n} \cdot \vec{v}_1)^2 (\hat{n} \cdot \vec{S}_1)^2 + 90 \hat{n} \cdot \vec{v}_1 \hat{n} \cdot \vec{v}_2 (\hat{n} \cdot \vec{S}_1)^2 + \frac{54}{7} \vec{v}_1 \cdot \vec{v}_1 (\hat{n} \cdot \vec{S}_1)^2 - \frac{90}{7} \vec{v}_1 \cdot \vec{v}_2 (\hat{n} \cdot \vec{S}_1)^2 + \right. \\ \left. \frac{216}{7} \hat{n} \cdot \vec{v}_1 \vec{S}_1 \cdot \vec{v}_1 \hat{n} \cdot \vec{S}_1 - \frac{180}{7} \hat{n} \cdot \vec{v}_2 \vec{S}_1 \cdot \vec{v}_1 \hat{n} \cdot \vec{S}_1 - \frac{180}{7} \hat{n} \cdot \vec{v}_1 \vec{S}_1 \cdot \vec{v}_2 \hat{n} \cdot \vec{S}_1 - \frac{108}{35} (\vec{S}_1 \cdot \vec{v}_1)^2 + \frac{54}{7} (\hat{n} \cdot \vec{v}_1)^2 \right. \\ \left. \vec{S}_1 \cdot \vec{S}_1 - \frac{90}{7} \hat{n} \cdot \vec{v}_1 \hat{n} \cdot \vec{v}_2 \vec{S}_1 \cdot \vec{S}_1 + \frac{36}{7} \vec{S}_1 \cdot \vec{v}_1 \vec{S}_1 \cdot \vec{v}_2 - \frac{54}{35} \vec{S}_1 \cdot \vec{S}_1 \vec{v}_1 \cdot \vec{v}_1 + \frac{18}{7} \vec{S}_1 \cdot \vec{S}_1 \vec{v}_1 \cdot \vec{v}_2 \right) \log \left( \frac{r}{R_\theta} \right) + \\ \frac{1}{\epsilon_d} \left( \frac{\frac{24}{5} (\hat{n} \cdot \vec{S}_1)^2 - \frac{8}{5} \vec{S}_1 \cdot \vec{S}_1}{r^3} + \frac{1}{r^4} \left( -24 \hat{n} \cdot \vec{S}_1 \hat{n} \cdot \vec{S}_1 \hat{n} \cdot \vec{v}_1 + \frac{24}{5} \vec{S}_1 \cdot \vec{S}_1 \hat{n} \cdot \vec{v}_1 + 24 \hat{n} \cdot \vec{S}_1 \hat{n} \cdot \vec{S}_1 \hat{n} \cdot \vec{v}_2 + \right. \right. \\ \left. \frac{24}{5} \hat{n} \cdot \vec{S}_1 \vec{S}_1 \cdot \vec{v}_1 - \frac{24}{5} \hat{n} \cdot \vec{S}_1 \vec{S}_1 \cdot \vec{v}_2 - \frac{24}{5} \hat{n} \cdot \vec{v}_2 \vec{S}_1 \cdot \vec{S}_1 + \frac{24}{5} \hat{n} \cdot \vec{S}_1 \vec{S}_1 \cdot \vec{v}_1 - \frac{24}{5} \hat{n} \cdot \vec{S}_1 \vec{S}_1 \cdot \vec{v}_2 \right) +$$

$$\left. \begin{aligned} & \frac{1}{r^5} \left( 18 (\hat{n} \cdot \vec{v}_1)^2 (\hat{n} \cdot \vec{S}_1)^2 - 30 \hat{n} \cdot \vec{v}_1 \hat{n} \cdot \vec{v}_2 (\hat{n} \cdot \vec{S}_1)^2 - \frac{18}{7} \vec{v}_1 \cdot \vec{v}_1 (\hat{n} \cdot \vec{S}_1)^2 + \frac{30}{7} \vec{v}_1 \cdot \vec{v}_2 (\hat{n} \cdot \vec{S}_1)^2 - \right. \\ & \left. \frac{72}{7} \hat{n} \cdot \vec{v}_1 \vec{S}_1 \cdot \vec{v}_1 \hat{n} \cdot \vec{S}_1 + \frac{60}{7} \hat{n} \cdot \vec{v}_2 \vec{S}_1 \cdot \vec{v}_1 \hat{n} \cdot \vec{S}_1 + \frac{60}{7} \hat{n} \cdot \vec{v}_1 \vec{S}_1 \cdot \vec{v}_2 \hat{n} \cdot \vec{S}_1 + \frac{36}{35} (\vec{S}_1 \cdot \vec{v}_1)^2 - \right. \\ & \left. \frac{18}{7} (\hat{n} \cdot \vec{v}_1)^2 \vec{S}_1 \cdot \vec{S}_1 + \frac{30}{7} \hat{n} \cdot \vec{v}_1 \hat{n} \cdot \vec{v}_2 \vec{S}_1 \cdot \vec{S}_1 - \frac{12}{7} \vec{S}_1 \cdot \vec{v}_1 \vec{S}_1 \cdot \vec{v}_2 + \frac{18}{35} \vec{S}_1 \cdot \vec{S}_1 \vec{v}_1 \cdot \vec{v}_1 - \frac{6}{7} \vec{S}_1 \cdot \vec{S}_1 \vec{v}_1 \cdot \vec{v}_2 \right) \Bigg\} \end{aligned}$$

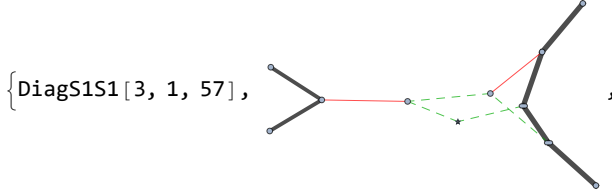

$$\begin{aligned} G^3 m_1 m_2 & \left( \frac{\frac{27}{25} \left( \hat{n} \cdot \vec{S}_1 \right)^2 - \frac{47}{75} \vec{S}_1 \cdot \vec{S}_1}{r^3} + \frac{1}{r^4} \left( -9 \hat{n} \cdot \vec{S}_1 \hat{n} \cdot \vec{S}_1 \hat{n} \cdot \vec{v}_1 + \frac{77}{25} \vec{S}_1 \cdot \vec{S}_1 \hat{n} \cdot \vec{v}_1 + 9 \hat{n} \cdot \vec{S}_1 \hat{n} \cdot \vec{S}_1 \hat{n} \cdot \vec{v}_2 + \right. \right. \\ & \left. \frac{7}{25} \hat{n} \cdot \vec{S}_1 \vec{S}_1 \cdot \vec{v}_1 - \frac{27}{25} \hat{n} \cdot \vec{S}_1 \vec{S}_1 \cdot \vec{v}_2 - \frac{77}{25} \hat{n} \cdot \vec{v}_2 \vec{S}_1 \cdot \vec{S}_1 + \frac{47}{25} \hat{n} \cdot \vec{S}_1 \vec{S}_1 \cdot \vec{v}_1 - \frac{27}{25} \hat{n} \cdot \vec{S}_1 \vec{S}_1 \cdot \vec{v}_2 \right) + \frac{1}{r^5} \\ & \left( -\frac{8}{7} (\hat{n} \cdot \vec{S}_1 \cdot \vec{v}_1)^2 + \frac{28}{3} (\hat{n} \cdot \vec{S}_1)^2 (\hat{n} \cdot \vec{v}_1)^2 - \frac{1844 (\vec{S}_1 \cdot \vec{v}_1)^2}{3675} - 13 (\hat{n} \cdot \vec{S}_1)^2 \hat{n} \cdot \vec{v}_1 \hat{n} \cdot \vec{v}_2 - \frac{496}{147} (\hat{n} \cdot \vec{v}_1)^2 \vec{S}_1 \cdot \vec{S}_1 + \right. \\ & \frac{171}{49} \hat{n} \cdot \vec{v}_1 \hat{n} \cdot \vec{v}_2 \vec{S}_1 \cdot \vec{S}_1 - \frac{388}{147} \hat{n} \cdot \vec{S}_1 \hat{n} \cdot \vec{v}_1 \vec{S}_1 \cdot \vec{v}_1 + \frac{62}{49} \hat{n} \cdot \vec{S}_1 \hat{n} \cdot \vec{v}_2 \vec{S}_1 \cdot \vec{v}_1 + \frac{146}{49} \hat{n} \cdot \vec{S}_1 \hat{n} \cdot \vec{v}_1 \vec{S}_1 \cdot \vec{v}_2 - \\ & \left. \frac{58 \vec{S}_1 \cdot \vec{v}_1 \vec{S}_1 \cdot \vec{v}_2}{1225} - \frac{160}{147} (\hat{n} \cdot \vec{S}_1)^2 \vec{v}_1 \cdot \vec{v}_1 + \frac{4748 \vec{S}_1 \cdot \vec{S}_1 \vec{v}_1 \cdot \vec{v}_1}{3675} + \frac{73}{49} (\hat{n} \cdot \vec{S}_1)^2 \vec{v}_1 \cdot \vec{v}_2 - \frac{729 \vec{S}_1 \cdot \vec{S}_1 \vec{v}_1 \cdot \vec{v}_2}{1225} \right) + \\ & \left( \frac{\frac{6}{5} \vec{S}_1 \cdot \vec{S}_1 - \frac{18}{5} (\hat{n} \cdot \vec{S}_1)^2}{r^3} + \frac{1}{r^4} \left( 18 \hat{n} \cdot \vec{S}_1 \hat{n} \cdot \vec{S}_1 \hat{n} \cdot \vec{v}_1 - \frac{18}{5} \vec{S}_1 \cdot \vec{S}_1 \hat{n} \cdot \vec{v}_1 - 18 \hat{n} \cdot \vec{S}_1 \hat{n} \cdot \vec{S}_1 \hat{n} \cdot \vec{v}_2 - \right. \right. \\ & \left. \frac{18}{5} \hat{n} \cdot \vec{S}_1 \vec{S}_1 \cdot \vec{v}_1 + \frac{18}{5} \hat{n} \cdot \vec{S}_1 \vec{S}_1 \cdot \vec{v}_2 + \frac{18}{5} \hat{n} \cdot \vec{v}_2 \vec{S}_1 \cdot \vec{S}_1 - \frac{18}{5} \hat{n} \cdot \vec{S}_1 \vec{S}_1 \cdot \vec{v}_1 + \frac{18}{5} \hat{n} \cdot \vec{S}_1 \vec{S}_1 \cdot \vec{v}_2 \right) + \frac{1}{r^5} \\ & \left( -12 (\hat{n} \cdot \vec{v}_1)^2 (\hat{n} \cdot \vec{S}_1)^2 + 18 \hat{n} \cdot \vec{v}_1 \hat{n} \cdot \vec{v}_2 (\hat{n} \cdot \vec{S}_1)^2 + \frac{12}{7} \vec{v}_1 \cdot \vec{v}_1 (\hat{n} \cdot \vec{S}_1)^2 - \frac{18}{7} \vec{v}_1 \cdot \vec{v}_2 (\hat{n} \cdot \vec{S}_1)^2 + \right. \\ & \frac{48}{7} \hat{n} \cdot \vec{v}_1 \vec{S}_1 \cdot \vec{v}_1 \hat{n} \cdot \vec{S}_1 - \frac{36}{7} \hat{n} \cdot \vec{v}_2 \vec{S}_1 \cdot \vec{v}_1 \hat{n} \cdot \vec{S}_1 - \frac{36}{7} \hat{n} \cdot \vec{v}_1 \vec{S}_1 \cdot \vec{v}_2 \hat{n} \cdot \vec{S}_1 - \frac{24}{35} (\vec{S}_1 \cdot \vec{v}_1)^2 + \frac{12}{7} (\hat{n} \cdot \vec{v}_1)^2 \vec{S}_1 \cdot \vec{S}_1 - \\ & \left. \frac{18}{7} \hat{n} \cdot \vec{v}_1 \hat{n} \cdot \vec{v}_2 \vec{S}_1 \cdot \vec{S}_1 + \frac{36}{35} \vec{S}_1 \cdot \vec{v}_1 \vec{S}_1 \cdot \vec{v}_2 - \frac{12}{35} \vec{S}_1 \cdot \vec{S}_1 \vec{v}_1 \cdot \vec{v}_1 + \frac{18}{35} \vec{S}_1 \cdot \vec{S}_1 \vec{v}_1 \cdot \vec{v}_2 \right) \log \left( \frac{r}{R_0} \right) + \\ & \frac{1}{\epsilon_d} \left( \frac{\frac{6}{5} (\hat{n} \cdot \vec{S}_1)^2 - \frac{2}{5} \vec{S}_1 \cdot \vec{S}_1}{r^3} + \frac{1}{r^4} \left( -6 \hat{n} \cdot \vec{S}_1 \hat{n} \cdot \vec{S}_1 \hat{n} \cdot \vec{v}_1 + \frac{6}{5} \vec{S}_1 \cdot \vec{S}_1 \hat{n} \cdot \vec{v}_1 + 6 \hat{n} \cdot \vec{S}_1 \hat{n} \cdot \vec{S}_1 \hat{n} \cdot \vec{v}_2 + \right. \right. \end{aligned}$$

$$\left. \begin{aligned} & \frac{6}{5} \hat{n} \cdot \vec{S}_1 \vec{S}_1^{\frac{1}{2}} \cdot \vec{v}_1 - \frac{6}{5} \hat{n} \cdot \vec{S}_1 \vec{S}_1^{\frac{1}{2}} \cdot \vec{v}_2 - \frac{6}{5} \hat{n} \cdot \vec{v}_2 \vec{S}_1 \cdot \vec{S}_1^{\frac{1}{2}} + \frac{6}{5} \hat{n} \cdot \vec{S}_1 \vec{S}_1^{\frac{1}{2}} \cdot \vec{v}_1 - \frac{6}{5} \hat{n} \cdot \vec{S}_1 \vec{S}_1^{\frac{1}{2}} \cdot \vec{v}_2 \Big) + \\ & \frac{1}{r^5} \left( 4 \left( \hat{n} \cdot \vec{v}_1 \right)^2 \left( \hat{n} \cdot \vec{S}_1 \right)^2 - 6 \hat{n} \cdot \vec{v}_1 \hat{n} \cdot \vec{v}_2 \left( \hat{n} \cdot \vec{S}_1 \right)^2 - \frac{4}{7} \vec{v}_1 \cdot \vec{v}_1 \left( \hat{n} \cdot \vec{S}_1 \right)^2 + \frac{6}{7} \vec{v}_1 \cdot \vec{v}_2 \left( \hat{n} \cdot \vec{S}_1 \right)^2 - \right. \\ & \left. \frac{16}{7} \hat{n} \cdot \vec{v}_1 \vec{S}_1 \cdot \vec{v}_1 \hat{n} \cdot \vec{S}_1 + \frac{12}{7} \hat{n} \cdot \vec{v}_2 \vec{S}_1 \cdot \vec{v}_1 \hat{n} \cdot \vec{S}_1 + \frac{12}{7} \hat{n} \cdot \vec{v}_1 \vec{S}_1 \cdot \vec{v}_2 \hat{n} \cdot \vec{S}_1 + \frac{8}{35} \left( \vec{S}_1 \cdot \vec{v}_1 \right)^2 - \right. \\ & \left. \frac{4}{7} \left( \hat{n} \cdot \vec{v}_1 \right)^2 \vec{S}_1 \cdot \vec{S}_1 + \frac{6}{7} \hat{n} \cdot \vec{v}_1 \hat{n} \cdot \vec{v}_2 \vec{S}_1 \cdot \vec{S}_1 - \frac{12}{35} \vec{S}_1 \cdot \vec{v}_1 \vec{S}_1 \cdot \vec{v}_2 + \frac{4}{35} \vec{S}_1 \cdot \vec{S}_1 \vec{v}_1 \cdot \vec{v}_1 - \frac{6}{35} \vec{S}_1 \cdot \vec{S}_1 \vec{v}_1 \cdot \vec{v}_2 \right) \Bigg) \Bigg\} \end{aligned}$$

{DiagS1S1[3, 1, 58],

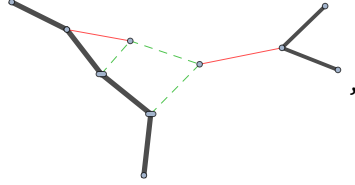

$$\begin{aligned} & G^3 m_1 m_2 \left( \frac{-\frac{24}{5} \vec{S}_1 \cdot \vec{a}_1 \hat{n} \cdot \vec{S}_1 + \frac{24}{5} \vec{S}_1 \cdot \vec{S}_1 \hat{n} \cdot \vec{a}_1 + \frac{24}{5} \vec{S}_1 \cdot \vec{S}_1^{\frac{1}{2}} \hat{n} \cdot \vec{v}_1 - \frac{24}{5} \hat{n} \cdot \vec{S}_1 \vec{S}_1^{\frac{1}{2}} \cdot \vec{v}_1}{r^4} + \right. \\ & \frac{1}{r^5} \left( \frac{32}{7} \left( \hat{n} \times \vec{S}_1 \cdot \vec{v}_1 \right)^2 - \frac{40}{7} \vec{S}_1 \cdot \vec{S}_1 \left( \hat{n} \cdot \vec{v}_1 \right)^2 + \frac{40}{7} \hat{n} \cdot \vec{S}_1 \hat{n} \cdot \vec{v}_1 \vec{S}_1 \cdot \vec{v}_1 + \frac{6}{7} \vec{v}_1 \cdot \vec{v}_1 \left( \hat{n} \cdot \vec{S}_1 \right)^2 + \right. \\ & \left. \left. \frac{6}{7} \vec{v}_2 \cdot \vec{v}_2 \left( \hat{n} \cdot \vec{S}_1 \right)^2 - \frac{32}{35} \left( \vec{S}_1 \cdot \vec{v}_1 \right)^2 + \frac{10}{7} \vec{S}_1 \cdot \vec{S}_1 \vec{v}_1 \cdot \vec{v}_1 + \frac{18}{35} \vec{S}_1 \cdot \vec{S}_1 \vec{v}_2 \cdot \vec{v}_2 \right) \right) \Bigg\} \end{aligned}$$

{DiagS1S1[3, 1, 59],

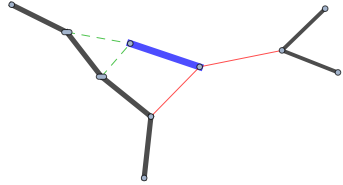

$$\begin{aligned} & \frac{-\frac{493}{98} \hat{n} \cdot \vec{S}_1^{\frac{1}{2}} \hat{n} \cdot \vec{S}_1 \hat{n} \cdot \vec{v}_1 - \frac{75}{98} \vec{S}_1 \cdot \vec{S}_1^{\frac{1}{2}} \hat{n} \cdot \vec{v}_1 + \frac{159}{245} \hat{n} \cdot \vec{S}_1 \vec{S}_1^{\frac{1}{2}} \cdot \vec{v}_1 + 2 \hat{n} \cdot \vec{S}_1 \vec{S}_1 \cdot \vec{a}_1 - 2 \hat{n} \cdot \vec{a}_1 \vec{S}_1 \cdot \vec{S}_1 + \frac{747}{245} \hat{n} \cdot \vec{S}_1 \vec{S}_1^{\frac{1}{2}} \cdot \vec{v}_1}{r^4} + \\ & \frac{1}{r^5} \left( -\frac{10}{7} \left( \hat{n} \times \vec{S}_1 \cdot \vec{v}_1 \right)^2 + \frac{251}{48} \left( \hat{n} \cdot \vec{S}_1 \right)^2 \left( \hat{n} \cdot \vec{v}_1 \right)^2 - \frac{19 \left( \vec{S}_1 \cdot \vec{v}_1 \right)^2}{5880} + \frac{1}{4} \left( \hat{n} \cdot \vec{S}_1 \right)^2 \hat{n} \cdot \vec{v}_1 \hat{n} \cdot \vec{v}_2 - \right. \\ & \frac{989 \left( \hat{n} \cdot \vec{v}_1 \right)^2 \vec{S}_1 \cdot \vec{S}_1}{2352} - \frac{13}{196} \hat{n} \cdot \vec{v}_1 \hat{n} \cdot \vec{v}_2 \vec{S}_1 \cdot \vec{S}_1 - \frac{1871}{588} \hat{n} \cdot \vec{S}_1 \hat{n} \cdot \vec{v}_1 \vec{S}_1 \cdot \vec{v}_1 - \frac{27}{98} \hat{n} \cdot \vec{S}_1 \hat{n} \cdot \vec{v}_2 \vec{S}_1 \cdot \vec{v}_1 - \\ & \frac{13}{98} \hat{n} \cdot \vec{S}_1 \hat{n} \cdot \vec{v}_1 \vec{S}_1 \cdot \vec{v}_2 + \frac{177 \vec{S}_1 \cdot \vec{v}_1 \vec{S}_1 \cdot \vec{v}_2}{2450} - \frac{989 \left( \hat{n} \cdot \vec{S}_1 \right)^2 \vec{v}_1 \cdot \vec{v}_1}{2352} + \frac{601 \vec{S}_1 \cdot \vec{S}_1 \vec{v}_1 \cdot \vec{v}_1}{2352} - \\ & \left. \frac{13}{196} \left( \hat{n} \cdot \vec{S}_1 \right)^2 \vec{v}_1 \cdot \vec{v}_2 + \frac{107 \vec{S}_1 \cdot \vec{S}_1 \vec{v}_1 \cdot \vec{v}_2}{4900} + \frac{15}{28} \left( \hat{n} \cdot \vec{S}_1 \right)^2 \vec{v}_2 \cdot \vec{v}_2 - \frac{39}{140} \vec{S}_1 \cdot \vec{S}_1 \vec{v}_2 \cdot \vec{v}_2 \right) + \\ & \left( \frac{\frac{3}{5} \vec{S}_1 \cdot \vec{S}_1^{\frac{1}{2}} - \frac{9}{5} \left( \hat{n} \cdot \vec{S}_1 \right)^2}{r^3} + \frac{\frac{30}{7} \hat{n} \cdot \vec{S}_1 \hat{n} \cdot \vec{S}_1 \hat{n} \cdot \vec{v}_1 - \frac{6}{7} \vec{S}_1 \cdot \vec{S}_1^{\frac{1}{2}} \hat{n} \cdot \vec{v}_1 - \frac{6}{7} \hat{n} \cdot \vec{S}_1 \vec{S}_1^{\frac{1}{2}} \cdot \vec{v}_1 - \frac{6}{7} \hat{n} \cdot \vec{S}_1 \vec{S}_1^{\frac{1}{2}} \cdot \vec{v}_1}{r^4} + \right. \end{aligned}$$

$$\begin{aligned}
& \frac{1}{r^5} \left( -\frac{15}{4} (\hat{n} \cdot \vec{v}_1)^2 (\hat{n} \cdot \vec{S}_1)^2 + \frac{3}{2} \hat{n} \cdot \vec{v}_1 \hat{n} \cdot \vec{v}_2 (\hat{n} \cdot \vec{S}_1)^2 + \frac{15}{28} \vec{v}_1 \cdot \vec{v}_1 (\hat{n} \cdot \vec{S}_1)^2 - \frac{3}{14} \vec{v}_1 \cdot \vec{v}_2 (\hat{n} \cdot \vec{S}_1)^2 + \right. \\
& \quad \frac{15}{7} \hat{n} \cdot \vec{v}_1 \vec{S}_1 \cdot \vec{v}_1 \hat{n} \cdot \vec{S}_1 - \frac{3}{7} \hat{n} \cdot \vec{v}_2 \vec{S}_1 \cdot \vec{v}_1 \hat{n} \cdot \vec{S}_1 - \frac{3}{7} \hat{n} \cdot \vec{v}_1 \vec{S}_1 \cdot \vec{v}_2 \hat{n} \cdot \vec{S}_1 - \frac{3}{14} (\vec{S}_1 \cdot \vec{v}_1)^2 + \frac{15}{28} (\hat{n} \cdot \vec{v}_1)^2 \vec{S}_1 \cdot \vec{S}_1 - \\
& \quad \left. \frac{3}{14} \hat{n} \cdot \vec{v}_1 \hat{n} \cdot \vec{v}_2 \vec{S}_1 \cdot \vec{S}_1 + \frac{3}{35} \vec{S}_1 \cdot \vec{v}_1 \vec{S}_1 \cdot \vec{v}_2 - \frac{3}{28} \vec{S}_1 \cdot \vec{S}_1 \vec{v}_1 \cdot \vec{v}_1 + \frac{3}{70} \vec{S}_1 \cdot \vec{S}_1 \vec{v}_1 \cdot \vec{v}_2 \right) \log \left( \frac{r}{R_\theta} \right) + \frac{1}{\epsilon_d} \\
& \left( \frac{\frac{3}{5} (\hat{n} \cdot \vec{S}_1)^2 - \frac{1}{5} \vec{S}_1 \cdot \vec{S}_1}{r^3} + \frac{-\frac{10}{7} \hat{n} \cdot \vec{S}_1 \hat{n} \cdot \vec{S}_1 \hat{n} \cdot \vec{v}_1 + \frac{2}{7} \vec{S}_1 \cdot \vec{S}_1 \hat{n} \cdot \vec{v}_1 + \frac{2}{7} \hat{n} \cdot \vec{S}_1 \vec{S}_1 \cdot \vec{v}_1 + \frac{2}{7} \hat{n} \cdot \vec{S}_1 \vec{S}_1 \cdot \vec{v}_1}{r^4} + \right. \\
& \quad \frac{1}{r^5} \left( \frac{5}{4} (\hat{n} \cdot \vec{v}_1)^2 (\hat{n} \cdot \vec{S}_1)^2 - \frac{1}{2} \hat{n} \cdot \vec{v}_1 \hat{n} \cdot \vec{v}_2 (\hat{n} \cdot \vec{S}_1)^2 - \frac{5}{28} \vec{v}_1 \cdot \vec{v}_1 (\hat{n} \cdot \vec{S}_1)^2 + \frac{1}{14} \vec{v}_1 \cdot \vec{v}_2 (\hat{n} \cdot \vec{S}_1)^2 - \right. \\
& \quad \frac{5}{7} \hat{n} \cdot \vec{v}_1 \vec{S}_1 \cdot \vec{v}_1 \hat{n} \cdot \vec{S}_1 + \frac{1}{7} \hat{n} \cdot \vec{v}_2 \vec{S}_1 \cdot \vec{v}_1 \hat{n} \cdot \vec{S}_1 + \frac{1}{7} \hat{n} \cdot \vec{v}_1 \vec{S}_1 \cdot \vec{v}_2 \hat{n} \cdot \vec{S}_1 + \frac{1}{14} (\vec{S}_1 \cdot \vec{v}_1)^2 - \frac{5}{28} (\hat{n} \cdot \vec{v}_1)^2 \vec{S}_1 \cdot \vec{S}_1 + \\
& \quad \left. \left. \frac{1}{14} \hat{n} \cdot \vec{v}_1 \hat{n} \cdot \vec{v}_2 \vec{S}_1 \cdot \vec{S}_1 - \frac{1}{35} \vec{S}_1 \cdot \vec{v}_1 \vec{S}_1 \cdot \vec{v}_2 + \frac{1}{28} \vec{S}_1 \cdot \vec{S}_1 \vec{v}_1 \cdot \vec{v}_1 - \frac{1}{70} \vec{S}_1 \cdot \vec{S}_1 \vec{v}_1 \cdot \vec{v}_2 \right) \right) \Bigg\}
\end{aligned}$$

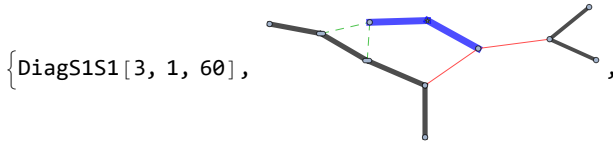

$$\begin{aligned}
& G^3 m_1 m_2 \left( \frac{1}{r^4} \left( -\frac{215}{98} \hat{n} \cdot \vec{S}_1 \hat{n} \cdot \vec{S}_1 \hat{n} \cdot \vec{v}_1 + \frac{1747 \vec{S}_1 \cdot \vec{S}_1 \hat{n} \cdot \vec{v}_1}{2450} + \frac{9}{2} \hat{n} \cdot \vec{S}_1 \hat{n} \cdot \vec{S}_1 \hat{n} \cdot \vec{v}_2 + \right. \right. \\
& \quad \left. \frac{907 \hat{n} \cdot \vec{S}_1 \vec{S}_1 \cdot \vec{v}_1}{2450} - \frac{21}{25} \hat{n} \cdot \vec{S}_1 \vec{S}_1 \cdot \vec{v}_2 - \frac{67}{50} \hat{n} \cdot \vec{v}_2 \vec{S}_1 \cdot \vec{S}_1 + \frac{907 \hat{n} \cdot \vec{S}_1 \vec{S}_1 \cdot \vec{v}_1}{2450} - \frac{21}{25} \hat{n} \cdot \vec{S}_1 \vec{S}_1 \cdot \vec{v}_2 \right) + \frac{1}{r^5} \\
& \quad \left( \frac{3}{14} (\hat{n} \cdot \vec{S}_1 \cdot \vec{v}_1)^2 + \frac{127}{48} (\hat{n} \cdot \vec{S}_1)^2 (\hat{n} \cdot \vec{v}_1)^2 + \frac{10313 (\vec{S}_1 \cdot \vec{v}_1)^2}{29400} - \frac{17}{2} (\hat{n} \cdot \vec{S}_1)^2 \hat{n} \cdot \vec{v}_1 \hat{n} \cdot \vec{v}_2 - \frac{601 (\hat{n} \cdot \vec{v}_1)^2 \vec{S}_1 \cdot \vec{S}_1}{2352} + \right. \\
& \quad \frac{81}{49} \hat{n} \cdot \vec{v}_1 \hat{n} \cdot \vec{v}_2 \vec{S}_1 \cdot \vec{S}_1 - \frac{1147}{588} \hat{n} \cdot \vec{S}_1 \hat{n} \cdot \vec{v}_1 \vec{S}_1 \cdot \vec{v}_1 + \frac{247}{98} \hat{n} \cdot \vec{S}_1 \hat{n} \cdot \vec{v}_2 \vec{S}_1 \cdot \vec{v}_1 + \frac{113}{49} \hat{n} \cdot \vec{S}_1 \hat{n} \cdot \vec{v}_1 \vec{S}_1 \cdot \vec{v}_2 - \\
& \quad \left. \frac{1151 \vec{S}_1 \cdot \vec{v}_1 \vec{S}_1 \cdot \vec{v}_2}{2450} - \frac{13 (\hat{n} \cdot \vec{S}_1)^2 \vec{v}_1 \cdot \vec{v}_1}{2352} - \frac{13207 \vec{S}_1 \cdot \vec{S}_1 \vec{v}_1 \cdot \vec{v}_1}{58800} + \frac{113}{98} (\hat{n} \cdot \vec{S}_1)^2 \vec{v}_1 \cdot \vec{v}_2 - \frac{384 \vec{S}_1 \cdot \vec{S}_1 \vec{v}_1 \cdot \vec{v}_2}{1225} \right) + \\
& \quad \left( \frac{1}{r^4} \left( \frac{9}{14} \hat{n} \cdot \vec{S}_1 \hat{n} \cdot \vec{S}_1 \hat{n} \cdot \vec{v}_1 - \frac{9}{70} \vec{S}_1 \cdot \vec{S}_1 \hat{n} \cdot \vec{v}_1 - \frac{3}{2} \hat{n} \cdot \vec{S}_1 \hat{n} \cdot \vec{S}_1 \hat{n} \cdot \vec{v}_2 - \frac{9}{70} \hat{n} \cdot \vec{S}_1 \vec{S}_1 \cdot \vec{v}_1 + \right. \right. \\
& \quad \left. \frac{3}{10} \hat{n} \cdot \vec{S}_1 \vec{S}_1 \cdot \vec{v}_2 + \frac{3}{10} \hat{n} \cdot \vec{v}_2 \vec{S}_1 \cdot \vec{S}_1 - \frac{9}{70} \hat{n} \cdot \vec{S}_1 \vec{S}_1 \cdot \vec{v}_1 + \frac{3}{10} \hat{n} \cdot \vec{S}_1 \vec{S}_1 \cdot \vec{v}_2 \right) + \frac{1}{r^5} \\
& \quad \left( -\frac{3}{4} (\hat{n} \cdot \vec{v}_1)^2 (\hat{n} \cdot \vec{S}_1)^2 + 3 \hat{n} \cdot \vec{v}_1 \hat{n} \cdot \vec{v}_2 (\hat{n} \cdot \vec{S}_1)^2 + \frac{3}{28} \vec{v}_1 \cdot \vec{v}_1 (\hat{n} \cdot \vec{S}_1)^2 - \frac{3}{7} \vec{v}_1 \cdot \vec{v}_2 (\hat{n} \cdot \vec{S}_1)^2 + \right. \\
& \quad \frac{3}{7} \hat{n} \cdot \vec{v}_1 \vec{S}_1 \cdot \vec{v}_1 \hat{n} \cdot \vec{S}_1 - \frac{6}{7} \hat{n} \cdot \vec{v}_2 \vec{S}_1 \cdot \vec{v}_1 \hat{n} \cdot \vec{S}_1 - \frac{6}{7} \hat{n} \cdot \vec{v}_1 \vec{S}_1 \cdot \vec{v}_2 \hat{n} \cdot \vec{S}_1 - \frac{3}{70} (\vec{S}_1 \cdot \vec{v}_1)^2 + \frac{3}{28} (\hat{n} \cdot \vec{v}_1)^2 \vec{S}_1 \cdot \vec{S}_1 - \\
& \quad \left. \left. \frac{3}{7} \hat{n} \cdot \vec{v}_1 \hat{n} \cdot \vec{v}_2 \vec{S}_1 \cdot \vec{S}_1 + \frac{6}{35} \vec{S}_1 \cdot \vec{v}_1 \vec{S}_1 \cdot \vec{v}_2 - \frac{3}{140} \vec{S}_1 \cdot \vec{S}_1 \vec{v}_1 \cdot \vec{v}_1 + \frac{3}{35} \vec{S}_1 \cdot \vec{S}_1 \vec{v}_1 \cdot \vec{v}_2 \right) \right) \log \left( \frac{r}{R_\theta} \right) +
\end{aligned}$$

$$\begin{aligned}
& \frac{1}{\epsilon_d} \left( \frac{1}{r^4} \left( -\frac{3}{14} \hat{n} \cdot \vec{S}_1 \hat{n} \cdot \vec{S}_1 \hat{n} \cdot \vec{v}_1 + \frac{3}{70} \vec{S}_1 \cdot \vec{S}_1 \hat{n} \cdot \vec{v}_1 + \frac{1}{2} \hat{n} \cdot \vec{S}_1 \hat{n} \cdot \vec{S}_1 \hat{n} \cdot \vec{v}_2 + \frac{3}{70} \hat{n} \cdot \vec{S}_1 \vec{S}_1 \cdot \vec{v}_1 - \right. \right. \\
& \quad \left. \frac{1}{10} \hat{n} \cdot \vec{S}_1 \vec{S}_1 \cdot \vec{v}_2 - \frac{1}{10} \hat{n} \cdot \vec{v}_2 \vec{S}_1 \cdot \vec{S}_1 + \frac{3}{70} \hat{n} \cdot \vec{S}_1 \vec{S}_1 \cdot \vec{v}_1 - \frac{1}{10} \hat{n} \cdot \vec{S}_1 \vec{S}_1 \cdot \vec{v}_2 \right) + \frac{1}{r^5} \\
& \quad \left( \frac{1}{4} (\hat{n} \cdot \vec{v}_1)^2 (\hat{n} \cdot \vec{S}_1)^2 - \hat{n} \cdot \vec{v}_1 \hat{n} \cdot \vec{v}_2 (\hat{n} \cdot \vec{S}_1)^2 - \frac{1}{28} \vec{v}_1 \cdot \vec{v}_1 (\hat{n} \cdot \vec{S}_1)^2 + \frac{1}{7} \vec{v}_1 \cdot \vec{v}_2 (\hat{n} \cdot \vec{S}_1)^2 - \right. \\
& \quad \left. \frac{1}{7} \hat{n} \cdot \vec{v}_1 \vec{S}_1 \cdot \vec{v}_1 \hat{n} \cdot \vec{S}_1 + \frac{2}{7} \hat{n} \cdot \vec{v}_2 \vec{S}_1 \cdot \vec{v}_1 \hat{n} \cdot \vec{S}_1 + \frac{2}{7} \hat{n} \cdot \vec{v}_1 \vec{S}_1 \cdot \vec{v}_2 \hat{n} \cdot \vec{S}_1 + \frac{1}{70} (\vec{S}_1 \cdot \vec{v}_1)^2 - \frac{1}{28} (\hat{n} \cdot \vec{v}_1)^2 \vec{S}_1 \cdot \vec{S}_1 + \right. \\
& \quad \left. \frac{1}{7} \hat{n} \cdot \vec{v}_1 \hat{n} \cdot \vec{v}_2 \vec{S}_1 \cdot \vec{S}_1 - \frac{2}{35} \vec{S}_1 \cdot \vec{v}_1 \vec{S}_1 \cdot \vec{v}_2 + \frac{1}{140} \vec{S}_1 \cdot \vec{S}_1 \vec{v}_1 \cdot \vec{v}_1 - \frac{1}{35} \vec{S}_1 \cdot \vec{S}_1 \vec{v}_1 \cdot \vec{v}_2 \right) \Bigg) \Bigg\}
\end{aligned}$$

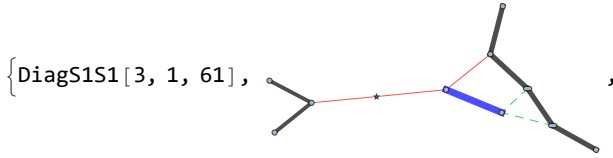

$$\begin{aligned}
& G^3 m_1 m_2 \left( \frac{-\frac{181}{98} \hat{n} \cdot \vec{S}_1 \hat{n} \cdot \vec{S}_1 \hat{n} \cdot \vec{v}_2 + \frac{251}{490} \vec{S}_1 \cdot \vec{S}_1 \hat{n} \cdot \vec{v}_2 + \frac{16}{49} \hat{n} \cdot \vec{S}_1 \vec{S}_1 \cdot \vec{v}_2 + \frac{16}{49} \hat{n} \cdot \vec{S}_1 \vec{S}_1 \cdot \vec{v}_2}{r^4} + \right. \\
& \quad \frac{1}{r^5} \left( 7 \hat{n} \cdot \vec{v}_1 \hat{n} \cdot \vec{v}_2 (\hat{n} \cdot \vec{S}_1)^2 - \frac{181}{196} \vec{v}_1 \cdot \vec{v}_2 (\hat{n} \cdot \vec{S}_1)^2 - \frac{181}{98} \hat{n} \cdot \vec{v}_2 \vec{S}_1 \cdot \vec{v}_1 \hat{n} \cdot \vec{S}_1 - \right. \\
& \quad \left. \frac{181}{98} \hat{n} \cdot \vec{v}_1 \vec{S}_1 \cdot \vec{v}_2 \hat{n} \cdot \vec{S}_1 - \frac{68}{49} \hat{n} \cdot \vec{v}_1 \hat{n} \cdot \vec{v}_2 \vec{S}_1 \cdot \vec{S}_1 + \frac{16}{49} \vec{S}_1 \cdot \vec{v}_1 \vec{S}_1 \cdot \vec{v}_2 + \frac{251}{980} \vec{S}_1 \cdot \vec{S}_1 \vec{v}_1 \cdot \vec{v}_2 \right) + \\
& \quad \left( \frac{\frac{15}{14} \hat{n} \cdot \vec{S}_1 \hat{n} \cdot \vec{S}_1 \hat{n} \cdot \vec{v}_2 - \frac{3}{14} \vec{S}_1 \cdot \vec{S}_1 \hat{n} \cdot \vec{v}_2 - \frac{3}{14} \hat{n} \cdot \vec{S}_1 \vec{S}_1 \cdot \vec{v}_2 - \frac{3}{14} \hat{n} \cdot \vec{S}_1 \vec{S}_1 \cdot \vec{v}_2}{r^4} + \frac{1}{r^5} \right. \\
& \quad \left( -\frac{15}{4} \hat{n} \cdot \vec{v}_1 \hat{n} \cdot \vec{v}_2 (\hat{n} \cdot \vec{S}_1)^2 + \frac{15}{28} \vec{v}_1 \cdot \vec{v}_2 (\hat{n} \cdot \vec{S}_1)^2 + \frac{15}{14} \hat{n} \cdot \vec{v}_2 \vec{S}_1 \cdot \vec{v}_1 \hat{n} \cdot \vec{S}_1 + \frac{15}{14} \hat{n} \cdot \vec{v}_1 \vec{S}_1 \cdot \vec{v}_2 \hat{n} \cdot \vec{S}_1 + \right. \\
& \quad \left. \frac{15}{28} \hat{n} \cdot \vec{v}_1 \hat{n} \cdot \vec{v}_2 \vec{S}_1 \cdot \vec{S}_1 - \frac{3}{14} \vec{S}_1 \cdot \vec{v}_1 \vec{S}_1 \cdot \vec{v}_2 - \frac{3}{28} \vec{S}_1 \cdot \vec{S}_1 \vec{v}_1 \cdot \vec{v}_2 \right) \log\left(\frac{r}{R_\theta}\right) + \\
& \quad \frac{1}{\epsilon_d} \left( \frac{-\frac{5}{14} \hat{n} \cdot \vec{S}_1 \hat{n} \cdot \vec{S}_1 \hat{n} \cdot \vec{v}_2 + \frac{1}{14} \vec{S}_1 \cdot \vec{S}_1 \hat{n} \cdot \vec{v}_2 + \frac{1}{14} \hat{n} \cdot \vec{S}_1 \vec{S}_1 \cdot \vec{v}_2 + \frac{1}{14} \hat{n} \cdot \vec{S}_1 \vec{S}_1 \cdot \vec{v}_2}{r^4} + \frac{1}{r^5} \right. \\
& \quad \left( \frac{5}{4} \hat{n} \cdot \vec{v}_1 \hat{n} \cdot \vec{v}_2 (\hat{n} \cdot \vec{S}_1)^2 - \frac{5}{28} \vec{v}_1 \cdot \vec{v}_2 (\hat{n} \cdot \vec{S}_1)^2 - \frac{5}{14} \hat{n} \cdot \vec{v}_2 \vec{S}_1 \cdot \vec{v}_1 \hat{n} \cdot \vec{S}_1 - \right. \\
& \quad \left. \frac{5}{14} \hat{n} \cdot \vec{v}_1 \vec{S}_1 \cdot \vec{v}_2 \hat{n} \cdot \vec{S}_1 - \frac{5}{28} \hat{n} \cdot \vec{v}_1 \hat{n} \cdot \vec{v}_2 \vec{S}_1 \cdot \vec{S}_1 + \frac{1}{14} \vec{S}_1 \cdot \vec{v}_1 \vec{S}_1 \cdot \vec{v}_2 + \frac{1}{28} \vec{S}_1 \cdot \vec{S}_1 \vec{v}_1 \cdot \vec{v}_2 \right) \Bigg) \Bigg\}
\end{aligned}$$

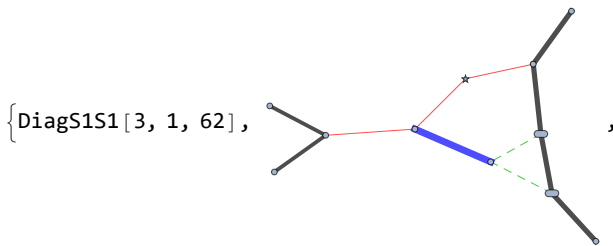

$$\begin{aligned}
& G^3 m_1 m_2 \left( \frac{-\frac{31}{98} \hat{n} \cdot \vec{S}_1 \hat{n} \cdot \vec{S}_1 \hat{n} \cdot \vec{v}_1 + \frac{421 \vec{S}_1 \cdot \vec{S}_1 \hat{n} \cdot \vec{v}_1}{2450} - \frac{17 \hat{n} \cdot \vec{S}_1 \vec{S}_1 \cdot \vec{v}_1}{1225} - \frac{17 \hat{n} \cdot \vec{S}_1 \vec{S}_1 \cdot \vec{v}_1}{1225}}{r^4} + \frac{1}{r^5} \right. \\
& \left( \frac{1}{7} (\hat{n} \times \vec{S}_1 \cdot \vec{v}_1)^2 + \frac{3}{16} (\hat{n} \cdot \vec{S}_1)^2 (\hat{n} \cdot \vec{v}_1)^2 + \frac{1089 (\vec{S}_1 \cdot \vec{v}_1)^2}{9800} - (\hat{n} \cdot \vec{S}_1)^2 \hat{n} \cdot \vec{v}_1 \hat{n} \cdot \vec{v}_2 + \frac{51}{784} (\hat{n} \cdot \vec{v}_1)^2 \vec{S}_1 \cdot \vec{S}_1 + \right. \\
& \frac{20}{49} \hat{n} \cdot \vec{v}_1 \hat{n} \cdot \vec{v}_2 \vec{S}_1 \cdot \vec{S}_1 - \frac{61}{196} \hat{n} \cdot \vec{S}_1 \hat{n} \cdot \vec{v}_1 \vec{S}_1 \cdot \vec{v}_1 - \frac{11}{98} \hat{n} \cdot \vec{S}_1 \hat{n} \cdot \vec{v}_2 \vec{S}_1 \cdot \vec{v}_1 + \frac{31}{98} \hat{n} \cdot \vec{S}_1 \hat{n} \cdot \vec{v}_1 \vec{S}_1 \cdot \vec{v}_2 + \\
& \left. \frac{17 \vec{S}_1 \cdot \vec{v}_1 \vec{S}_1 \cdot \vec{v}_2}{1225} + \frac{247}{784} (\hat{n} \cdot \vec{S}_1)^2 \vec{v}_1 \cdot \vec{v}_1 - \frac{4371 \vec{S}_1 \cdot \vec{S}_1 \vec{v}_1 \cdot \vec{v}_1}{19600} + \frac{31}{196} (\hat{n} \cdot \vec{S}_1)^2 \vec{v}_1 \cdot \vec{v}_2 - \frac{421 \vec{S}_1 \cdot \vec{S}_1 \vec{v}_1 \cdot \vec{v}_2}{4900} \right) + \\
& \left( \frac{-\frac{3}{14} \hat{n} \cdot \vec{S}_1 \hat{n} \cdot \vec{S}_1 \hat{n} \cdot \vec{v}_1 + \frac{3}{70} \vec{S}_1 \cdot \vec{S}_1 \hat{n} \cdot \vec{v}_1 + \frac{3}{70} \hat{n} \cdot \vec{S}_1 \vec{S}_1 \cdot \vec{v}_1 + \frac{3}{70} \hat{n} \cdot \vec{S}_1 \vec{S}_1 \cdot \vec{v}_1}}{r^4} + \frac{1}{r^5} \right. \\
& \left( \frac{3}{4} (\hat{n} \cdot \vec{v}_1)^2 (\hat{n} \cdot \vec{S}_1)^2 - \frac{3}{4} \hat{n} \cdot \vec{v}_1 \hat{n} \cdot \vec{v}_2 (\hat{n} \cdot \vec{S}_1)^2 - \frac{3}{28} \vec{v}_1 \cdot \vec{v}_1 (\hat{n} \cdot \vec{S}_1)^2 + \frac{3}{28} \vec{v}_1 \cdot \vec{v}_2 (\hat{n} \cdot \vec{S}_1)^2 - \right. \\
& \frac{3}{7} \hat{n} \cdot \vec{v}_1 \vec{S}_1 \cdot \vec{v}_1 \hat{n} \cdot \vec{S}_1 + \frac{3}{14} \hat{n} \cdot \vec{v}_2 \vec{S}_1 \cdot \vec{v}_1 \hat{n} \cdot \vec{S}_1 + \frac{3}{14} \hat{n} \cdot \vec{v}_1 \vec{S}_1 \cdot \vec{v}_2 \hat{n} \cdot \vec{S}_1 + \frac{3}{70} (\vec{S}_1 \cdot \vec{v}_1)^2 - \frac{3}{28} (\hat{n} \cdot \vec{v}_1)^2 \vec{S}_1 \cdot \vec{S}_1 + \\
& \left. \frac{3}{28} \hat{n} \cdot \vec{v}_1 \hat{n} \cdot \vec{v}_2 \vec{S}_1 \cdot \vec{S}_1 - \frac{3}{70} \vec{S}_1 \cdot \vec{v}_1 \vec{S}_1 \cdot \vec{v}_2 + \frac{3}{140} \vec{S}_1 \cdot \vec{S}_1 \vec{v}_1 \cdot \vec{v}_1 - \frac{3}{140} \vec{S}_1 \cdot \vec{S}_1 \vec{v}_1 \cdot \vec{v}_2 \right) \log\left(\frac{r}{R_0}\right) + \\
& \frac{1}{\epsilon_d} \left( \frac{\frac{1}{14} \hat{n} \cdot \vec{S}_1 \hat{n} \cdot \vec{S}_1 \hat{n} \cdot \vec{v}_1 - \frac{1}{70} \vec{S}_1 \cdot \vec{S}_1 \hat{n} \cdot \vec{v}_1 - \frac{1}{70} \hat{n} \cdot \vec{S}_1 \vec{S}_1 \cdot \vec{v}_1 - \frac{1}{70} \hat{n} \cdot \vec{S}_1 \vec{S}_1 \cdot \vec{v}_1}}{r^4} + \frac{1}{r^5} \right. \\
& \left( -\frac{1}{4} (\hat{n} \cdot \vec{v}_1)^2 (\hat{n} \cdot \vec{S}_1)^2 + \frac{1}{4} \hat{n} \cdot \vec{v}_1 \hat{n} \cdot \vec{v}_2 (\hat{n} \cdot \vec{S}_1)^2 + \frac{1}{28} \vec{v}_1 \cdot \vec{v}_1 (\hat{n} \cdot \vec{S}_1)^2 - \frac{1}{28} \vec{v}_1 \cdot \vec{v}_2 (\hat{n} \cdot \vec{S}_1)^2 + \right. \\
& \frac{1}{7} \hat{n} \cdot \vec{v}_1 \vec{S}_1 \cdot \vec{v}_1 \hat{n} \cdot \vec{S}_1 - \frac{1}{14} \hat{n} \cdot \vec{v}_2 \vec{S}_1 \cdot \vec{v}_1 \hat{n} \cdot \vec{S}_1 - \frac{1}{14} \hat{n} \cdot \vec{v}_1 \vec{S}_1 \cdot \vec{v}_2 \hat{n} \cdot \vec{S}_1 - \frac{1}{70} (\vec{S}_1 \cdot \vec{v}_1)^2 + \frac{1}{28} (\hat{n} \cdot \vec{v}_1)^2 \vec{S}_1 \cdot \vec{S}_1 - \\
& \left. \frac{1}{28} \hat{n} \cdot \vec{v}_1 \hat{n} \cdot \vec{v}_2 \vec{S}_1 \cdot \vec{S}_1 + \frac{1}{70} \vec{S}_1 \cdot \vec{v}_1 \vec{S}_1 \cdot \vec{v}_2 - \frac{1}{140} \vec{S}_1 \cdot \vec{S}_1 \vec{v}_1 \cdot \vec{v}_1 + \frac{1}{140} \vec{S}_1 \cdot \vec{S}_1 \vec{v}_1 \cdot \vec{v}_2 \right) \Bigg) \Bigg\}
\end{aligned}$$

{DiagS1S1[3, 1, 63],

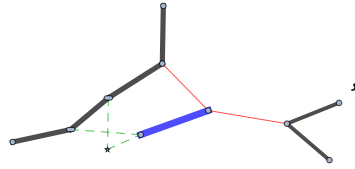

$$\begin{aligned}
& G^3 m_1 m_2 \left( \frac{\frac{43}{75} \vec{S}_1 \cdot \vec{S}_1 - \frac{13}{25} (\hat{n} \cdot \vec{S}_1)^2}{r^3} + \frac{1}{r^4} \left( 2 \hat{n} \cdot \vec{S}_1 \hat{n} \cdot \vec{S}_1 \hat{n} \cdot \vec{v}_1 - \frac{38}{25} \vec{S}_1 \cdot \vec{S}_1 \hat{n} \cdot \vec{v}_1 - 2 \hat{n} \cdot \vec{S}_1 \hat{n} \cdot \vec{S}_1 \hat{n} \cdot \vec{v}_2 - \right. \right. \\
& \left. \frac{11}{50} \hat{n} \cdot \vec{S}_1 \vec{S}_1 \cdot \vec{v}_1 + \frac{13}{25} \hat{n} \cdot \vec{S}_1 \vec{S}_1 \cdot \vec{v}_2 + \frac{38}{25} \hat{n} \cdot \vec{v}_2 \vec{S}_1 \cdot \vec{S}_1 - \frac{41}{50} \hat{n} \cdot \vec{S}_1 \vec{S}_1 \cdot \vec{v}_1 + \frac{13}{25} \hat{n} \cdot \vec{S}_1 \vec{S}_1 \cdot \vec{v}_2 \right) + \frac{1}{r^5} \\
& \left( -\frac{1}{7} (\hat{n} \times \vec{S}_1 \cdot \vec{v}_1)^2 - \frac{85}{24} (\hat{n} \cdot \vec{S}_1)^2 (\hat{n} \cdot \vec{v}_1)^2 - \frac{653 (\vec{S}_1 \cdot \vec{v}_1)^2}{14700} + 6 (\hat{n} \cdot \vec{S}_1)^2 \hat{n} \cdot \vec{v}_1 \hat{n} \cdot \vec{v}_2 + \frac{1063 (\hat{n} \cdot \vec{v}_1)^2 \vec{S}_1 \cdot \vec{S}_1}{1176} - \right.
\end{aligned}$$

$$\begin{aligned}
& \frac{127}{98} \hat{n} \cdot \vec{v}_1 \hat{n} \cdot \vec{v}_2 \vec{S}_1 \cdot \vec{S}_1 + \frac{164}{147} \hat{n} \cdot \vec{S}_1 \hat{n} \cdot \vec{v}_1 \vec{S}_1 \cdot \vec{v}_1 - \frac{79}{98} \hat{n} \cdot \vec{S}_1 \hat{n} \cdot \vec{v}_2 \vec{S}_1 \cdot \vec{v}_1 - \frac{78}{49} \hat{n} \cdot \vec{S}_1 \hat{n} \cdot \vec{v}_1 \vec{S}_1 \cdot \vec{v}_2 + \\
& \frac{311 \vec{S}_1 \cdot \vec{v}_1 \vec{S}_1 \cdot \vec{v}_2}{2450} + \frac{727 \left( \hat{n} \cdot \vec{S}_1 \right)^2 \vec{v}_1 \cdot \vec{v}_1}{1176} - \frac{6743 \vec{S}_1 \cdot \vec{S}_1 \vec{v}_1 \cdot \vec{v}_1}{29400} - \frac{39}{49} \left( \hat{n} \cdot \vec{S}_1 \right)^2 \vec{v}_1 \cdot \vec{v}_2 + \frac{593 \vec{S}_1 \cdot \vec{S}_1 \vec{v}_1 \cdot \vec{v}_2}{2450} \Bigg) + \\
& \left( \frac{\frac{1}{5} \vec{S}_1 \cdot \vec{S}_1 - \frac{3}{5} \left( \hat{n} \cdot \vec{S}_1 \right)^2}{r^3} + \frac{1}{r^4} \left( 3 \hat{n} \cdot \vec{S}_1 \hat{n} \cdot \vec{S}_1 \hat{n} \cdot \vec{v}_1 - \frac{3}{5} \vec{S}_1 \cdot \vec{S}_1 \hat{n} \cdot \vec{v}_1 - 3 \hat{n} \cdot \vec{S}_1 \hat{n} \cdot \vec{S}_1 \hat{n} \cdot \vec{v}_2 - \right. \right. \\
& \left. \frac{3}{5} \hat{n} \cdot \vec{S}_1 \vec{S}_1 \cdot \vec{v}_1 + \frac{3}{5} \hat{n} \cdot \vec{S}_1 \vec{S}_1 \cdot \vec{v}_2 + \frac{3}{5} \hat{n} \cdot \vec{v}_2 \vec{S}_1 \cdot \vec{S}_1 - \frac{3}{5} \hat{n} \cdot \vec{S}_1 \vec{S}_1 \cdot \vec{v}_1 + \frac{3}{5} \hat{n} \cdot \vec{S}_1 \vec{S}_1 \cdot \vec{v}_2 \right) + \frac{1}{r^5} \\
& \left( \frac{3}{2} \left( \hat{n} \cdot \vec{v}_1 \right)^2 \left( \hat{n} \cdot \vec{S}_1 \right)^2 - 3 \hat{n} \cdot \vec{v}_1 \hat{n} \cdot \vec{v}_2 \left( \hat{n} \cdot \vec{S}_1 \right)^2 - \frac{3}{14} \vec{v}_1 \cdot \vec{v}_1 \left( \hat{n} \cdot \vec{S}_1 \right)^2 + \frac{3}{7} \vec{v}_1 \cdot \vec{v}_2 \left( \hat{n} \cdot \vec{S}_1 \right)^2 - \right. \\
& \left. \frac{6}{7} \hat{n} \cdot \vec{v}_1 \vec{S}_1 \cdot \vec{v}_1 \hat{n} \cdot \vec{S}_1 + \frac{6}{7} \hat{n} \cdot \vec{v}_2 \vec{S}_1 \cdot \vec{v}_1 \hat{n} \cdot \vec{S}_1 + \frac{6}{7} \hat{n} \cdot \vec{v}_1 \vec{S}_1 \cdot \vec{v}_2 \hat{n} \cdot \vec{S}_1 + \frac{3}{35} \left( \vec{S}_1 \cdot \vec{v}_1 \right)^2 - \frac{3}{14} \left( \hat{n} \cdot \vec{v}_1 \right)^2 \vec{S}_1 \cdot \vec{S}_1 + \right. \\
& \left. \frac{3}{7} \hat{n} \cdot \vec{v}_1 \hat{n} \cdot \vec{v}_2 \vec{S}_1 \cdot \vec{S}_1 - \frac{6}{35} \vec{S}_1 \cdot \vec{v}_1 \vec{S}_1 \cdot \vec{v}_2 + \frac{3}{70} \vec{S}_1 \cdot \vec{S}_1 \vec{v}_1 \cdot \vec{v}_1 - \frac{3}{35} \vec{S}_1 \cdot \vec{S}_1 \vec{v}_1 \cdot \vec{v}_2 \right) \log \left( \frac{r}{R_0} \right) + \\
& \frac{1}{\epsilon_d} \left( \frac{\frac{1}{5} \left( \hat{n} \cdot \vec{S}_1 \right)^2 - \frac{1}{15} \vec{S}_1 \cdot \vec{S}_1}{r^3} + \frac{1}{r^4} \left( - \left( \hat{n} \cdot \vec{S}_1 \right) \hat{n} \cdot \vec{S}_1 \hat{n} \cdot \vec{v}_1 + \frac{1}{5} \vec{S}_1 \cdot \vec{S}_1 \hat{n} \cdot \vec{v}_1 + \hat{n} \cdot \vec{S}_1 \hat{n} \cdot \vec{S}_1 \hat{n} \cdot \vec{v}_2 + \right. \right. \\
& \left. \frac{1}{5} \hat{n} \cdot \vec{S}_1 \vec{S}_1 \cdot \vec{v}_1 - \frac{1}{5} \hat{n} \cdot \vec{S}_1 \vec{S}_1 \cdot \vec{v}_2 - \frac{1}{5} \hat{n} \cdot \vec{v}_2 \vec{S}_1 \cdot \vec{S}_1 + \frac{1}{5} \hat{n} \cdot \vec{S}_1 \vec{S}_1 \cdot \vec{v}_1 - \frac{1}{5} \hat{n} \cdot \vec{S}_1 \vec{S}_1 \cdot \vec{v}_2 \right) + \\
& \frac{1}{r^5} \left( - \frac{1}{2} \left( \hat{n} \cdot \vec{v}_1 \right)^2 \left( \hat{n} \cdot \vec{S}_1 \right)^2 + \hat{n} \cdot \vec{v}_1 \hat{n} \cdot \vec{v}_2 \left( \hat{n} \cdot \vec{S}_1 \right)^2 + \frac{1}{14} \vec{v}_1 \cdot \vec{v}_1 \left( \hat{n} \cdot \vec{S}_1 \right)^2 - \frac{1}{7} \vec{v}_1 \cdot \vec{v}_2 \left( \hat{n} \cdot \vec{S}_1 \right)^2 + \right. \\
& \left. \frac{2}{7} \hat{n} \cdot \vec{v}_1 \vec{S}_1 \cdot \vec{v}_1 \hat{n} \cdot \vec{S}_1 - \frac{2}{7} \hat{n} \cdot \vec{v}_2 \vec{S}_1 \cdot \vec{v}_1 \hat{n} \cdot \vec{S}_1 - \frac{2}{7} \hat{n} \cdot \vec{v}_1 \vec{S}_1 \cdot \vec{v}_2 \hat{n} \cdot \vec{S}_1 - \frac{1}{35} \left( \vec{S}_1 \cdot \vec{v}_1 \right)^2 + \right. \\
& \left. \frac{1}{14} \left( \hat{n} \cdot \vec{v}_1 \right)^2 \vec{S}_1 \cdot \vec{S}_1 - \frac{1}{7} \hat{n} \cdot \vec{v}_1 \hat{n} \cdot \vec{v}_2 \vec{S}_1 \cdot \vec{S}_1 + \frac{2}{35} \vec{S}_1 \cdot \vec{v}_1 \vec{S}_1 \cdot \vec{v}_2 - \frac{1}{70} \vec{S}_1 \cdot \vec{S}_1 \vec{v}_1 \cdot \vec{v}_1 + \frac{1}{35} \vec{S}_1 \cdot \vec{S}_1 \vec{v}_1 \cdot \vec{v}_2 \right) \Bigg) \Bigg\}
\end{aligned}$$

$\{ \text{DiagS1S1}[3, 2, 1],$ 
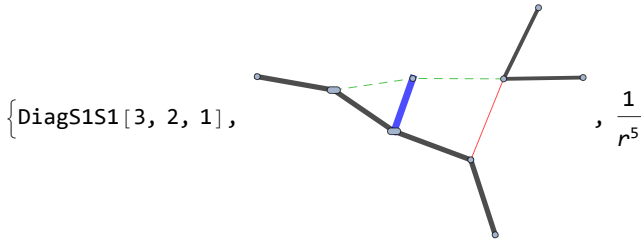
 $, \frac{1}{r^5}$

$$G^3 m_1 m_2 \left( 2 \vec{v}_1 \cdot \vec{v}_2 \left( \hat{n} \cdot \vec{S}_1 \right)^2 - 6 \hat{n} \cdot \vec{S}_1 \hat{n} \cdot \vec{v}_2 \vec{S}_1 \cdot \vec{v}_1 - 4 \hat{n} \cdot \vec{S}_1 \hat{n} \cdot \vec{v}_1 \vec{S}_1 \cdot \vec{v}_2 + \right. \\
\left. 10 \vec{S}_1 \cdot \vec{S}_1 \hat{n} \cdot \vec{v}_1 \hat{n} \cdot \vec{v}_2 + 3 \vec{S}_1 \cdot \vec{v}_1 \vec{S}_1 \cdot \vec{v}_2 - 3 \vec{S}_1 \cdot \vec{S}_1 \vec{v}_1 \cdot \vec{v}_2 \right) \Big\}$$

$$\left\{ \text{DiagS1S1}[3, 2, 2], \frac{1}{r^5} \right\}$$
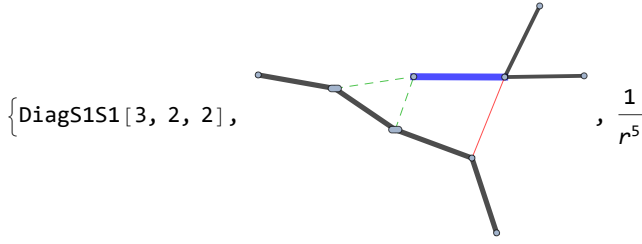

$$G^3 m_1 m_2 \left( -3 \left( \hat{n} \times \vec{S}_1 \cdot \vec{v}_2 \right)^2 + \frac{27}{4} \left( \hat{n} \cdot \vec{S}_1 \right)^2 \left( \hat{n} \cdot \vec{v}_2 \right)^2 - \frac{21}{4} \vec{S}_1 \cdot \vec{S}_1 \left( \hat{n} \cdot \vec{v}_2 \right)^2 + \right. \\ \left. 3 \hat{n} \cdot \vec{S}_1 \hat{n} \cdot \vec{v}_2 \vec{S}_1 \cdot \vec{v}_2 - \frac{21}{4} \vec{v}_2 \cdot \vec{v}_2 \left( \hat{n} \cdot \vec{S}_1 \right)^2 - 3 \left( \vec{S}_1 \cdot \vec{v}_2 \right)^2 + \frac{15}{4} \vec{S}_1 \cdot \vec{S}_1 \vec{v}_2 \cdot \vec{v}_2 \right) \Bigg\}$$

$$\left\{ \text{DiagS1S1}[3, 2, 3], G^3 m_1 m_2 \left( \frac{\vec{S}_1 \cdot \vec{a}_2 \hat{n} \cdot \vec{S}_1 - \vec{S}_1 \cdot \vec{S}_1 \hat{n} \cdot \vec{a}_2 - 2 \hat{n} \cdot \vec{S}_1 \hat{n} \cdot \vec{S}_1 \hat{n} \cdot \vec{v}_2}{r^4} + \frac{1}{r^5} \right. \right.$$
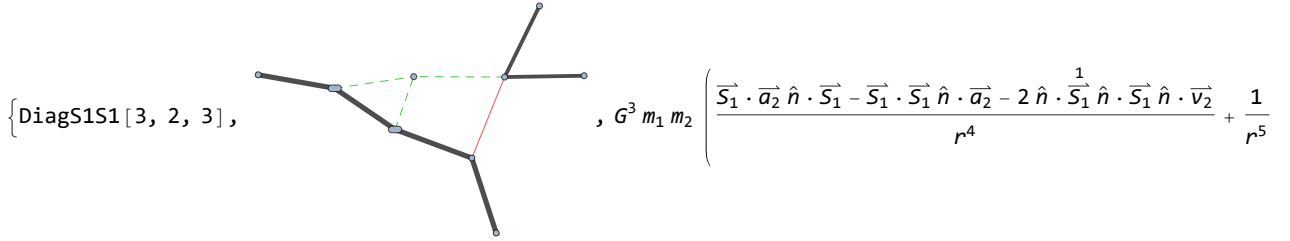

$$\left( 2 \hat{n} \times \vec{S}_1 \cdot \vec{v}_1 \hat{n} \times \vec{S}_1 \cdot \vec{v}_2 + \frac{9}{2} \left( \hat{n} \cdot \vec{S}_1 \right)^2 \hat{n} \cdot \vec{v}_1 \hat{n} \cdot \vec{v}_2 - \frac{3}{2} \vec{v}_1 \cdot \vec{v}_2 \left( \hat{n} \cdot \vec{S}_1 \right)^2 - \hat{n} \cdot \vec{S}_1 \hat{n} \cdot \vec{v}_2 \vec{S}_1 \cdot \vec{v}_1 + 5 \hat{n} \cdot \vec{S}_1 \hat{n} \cdot \vec{v}_2 \vec{S}_1 \cdot \vec{v}_2 - \right. \\ \left. 5 \vec{S}_1 \cdot \vec{S}_1 \left( \hat{n} \cdot \vec{v}_2 \right)^2 - \frac{1}{2} \vec{S}_1 \cdot \vec{S}_1 \hat{n} \cdot \vec{v}_1 \hat{n} \cdot \vec{v}_2 - \left( \vec{S}_1 \cdot \vec{v}_2 \right)^2 + \frac{1}{2} \vec{S}_1 \cdot \vec{S}_1 \vec{v}_1 \cdot \vec{v}_2 + \vec{S}_1 \cdot \vec{S}_1 \vec{v}_2 \cdot \vec{v}_2 \right) \Bigg\}$$

$$\left\{ \text{DiagS1S1}[3, 2, 4], \right.$$
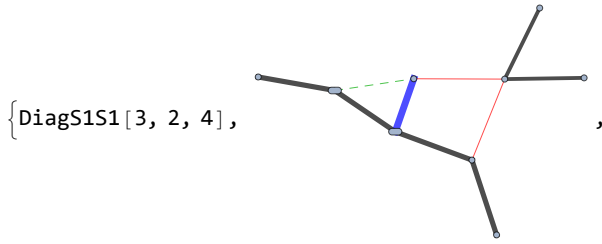

$$G^3 m_1 m_2 \left( \frac{1}{r^5} \left( -2 \left( \hat{n} \times \vec{S}_1 \cdot \vec{v}_1 \right)^2 + 14 \left( \hat{n} \cdot \vec{S}_1 \right)^2 \left( \hat{n} \cdot \vec{v}_1 \right)^2 - 14 \left( \hat{n} \cdot \vec{S}_1 \right)^2 \hat{n} \cdot \vec{v}_1 \hat{n} \cdot \vec{v}_2 + 8 \vec{S}_1 \cdot \vec{S}_1 \left( \hat{n} \cdot \vec{v}_1 \right)^2 - \right. \right. \\ \left. 10 \vec{S}_1 \cdot \vec{S}_1 \hat{n} \cdot \vec{v}_1 \hat{n} \cdot \vec{v}_2 - 12 \hat{n} \cdot \vec{S}_1 \hat{n} \cdot \vec{v}_1 \vec{S}_1 \cdot \vec{v}_1 + 10 \hat{n} \cdot \vec{S}_1 \hat{n} \cdot \vec{v}_2 \vec{S}_1 \cdot \vec{v}_1 + 4 \hat{n} \cdot \vec{S}_1 \hat{n} \cdot \vec{v}_1 \vec{S}_1 \cdot \vec{v}_2 - \right. \\ \left. 2 \vec{v}_1 \cdot \vec{v}_1 \left( \hat{n} \cdot \vec{S}_1 \right)^2 + 2 \vec{v}_1 \cdot \vec{v}_2 \left( \hat{n} \cdot \vec{S}_1 \right)^2 + \left( \vec{S}_1 \cdot \vec{v}_1 \right)^2 - 2 \vec{S}_1 \cdot \vec{v}_1 \vec{S}_1 \cdot \vec{v}_2 - \vec{S}_1 \cdot \vec{S}_1 \vec{v}_1 \cdot \vec{v}_1 + 2 \vec{S}_1 \cdot \vec{S}_1 \vec{v}_1 \cdot \vec{v}_2 \right) + \\ \left. \frac{-4 \hat{n} \cdot \vec{S}_1 \hat{n} \cdot \vec{S}_1 \hat{n} \cdot \vec{v}_1 - 3 \vec{S}_1 \cdot \vec{S}_1 \hat{n} \cdot \vec{v}_1 + \hat{n} \cdot \vec{S}_1 \vec{S}_1 \cdot \vec{v}_1 + 2 \hat{n} \cdot \vec{S}_1 \vec{S}_1 \cdot \vec{v}_1}{r^4} \right) \Bigg\}$$

$$\left\{ \text{DiagS1S1}[3, 2, 5], -\frac{4 G^3 m_1 m_2 \left( \hat{n} \times \vec{S}_1 \cdot \vec{v}_1 \right)^2}{r^5} \right\}$$
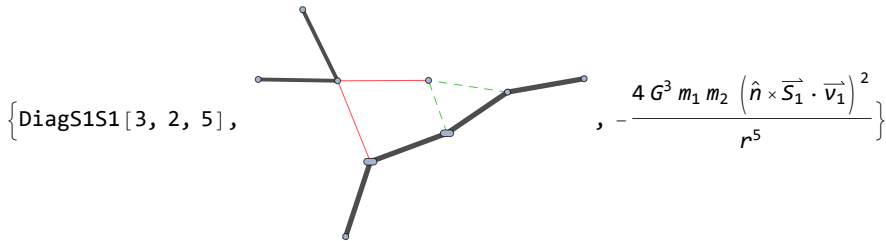

$\{\text{DiagS1S1}[3, 2, 6],$ 
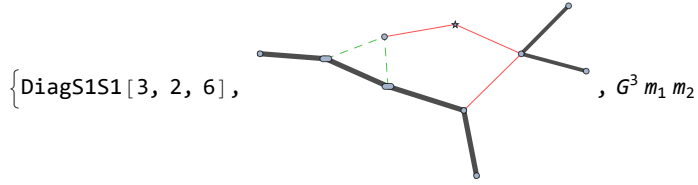
 $, G^3 m_1 m_2$

$$\left\{ \frac{1}{r^5} \left( (\hat{n} \cdot \vec{S}_1)^2 (-\hat{n} \cdot \vec{v}_1)^2 + 7 (\hat{n} \cdot \vec{S}_1)^2 \hat{n} \cdot \vec{v}_1 \hat{n} \cdot \vec{v}_2 - \vec{v}_1 \cdot \vec{v}_2 (\hat{n} \cdot \vec{S}_1)^2 + \frac{1}{2} \hat{n} \cdot \vec{S}_1 \hat{n} \cdot \vec{v}_1 \vec{S}_1 \cdot \vec{v}_1 - \frac{5}{2} \hat{n} \cdot \vec{S}_1 \hat{n} \cdot \vec{v}_2 \vec{S}_1 \cdot \vec{v}_1 - \right. \right.$$

$$\left. \left. 2 \hat{n} \cdot \vec{S}_1 \hat{n} \cdot \vec{v}_1 \vec{S}_1 \cdot \vec{v}_2 + \frac{1}{2} \vec{S}_1 \cdot \vec{S}_1 (\hat{n} \cdot \vec{v}_1)^2 - \frac{5}{2} \vec{S}_1 \cdot \vec{S}_1 \hat{n} \cdot \vec{v}_1 \hat{n} \cdot \vec{v}_2 + \frac{1}{2} \vec{S}_1 \cdot \vec{v}_1 \vec{S}_1 \cdot \vec{v}_2 + \frac{1}{2} \vec{S}_1 \cdot \vec{S}_1 \vec{v}_1 \cdot \vec{v}_2 \right) + \right.$$

$$\left. \frac{\frac{1}{2} \hat{n} \cdot \vec{S}_1 \hat{n} \cdot \vec{S}_1 \hat{n} \cdot \vec{v}_1 - \frac{1}{2} \vec{S}_1 \cdot \vec{S}_1 \hat{n} \cdot \vec{v}_1 - \frac{5}{2} \hat{n} \cdot \vec{S}_1 \hat{n} \cdot \vec{S}_1 \hat{n} \cdot \vec{v}_2 + \frac{1}{2} \hat{n} \cdot \vec{S}_1 \vec{S}_1 \cdot \vec{v}_2 + \frac{3}{2} \vec{S}_1 \cdot \vec{S}_1 \hat{n} \cdot \vec{v}_2 + \frac{1}{2} \hat{n} \cdot \vec{S}_1 \vec{S}_1 \cdot \vec{v}_2}{r^4} \right\}$$

$\{\text{DiagS1S1}[3, 2, 7],$ 
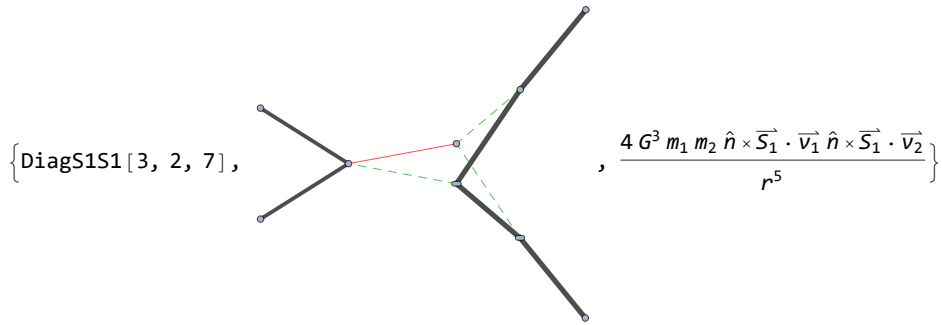
 $, \frac{4 G^3 m_1 m_2 \hat{n} \times \vec{S}_1 \cdot \vec{v}_1 \hat{n} \times \vec{S}_1 \cdot \vec{v}_2}{r^5} \}$

$\{\text{DiagS1S1}[3, 2, 8],$ 
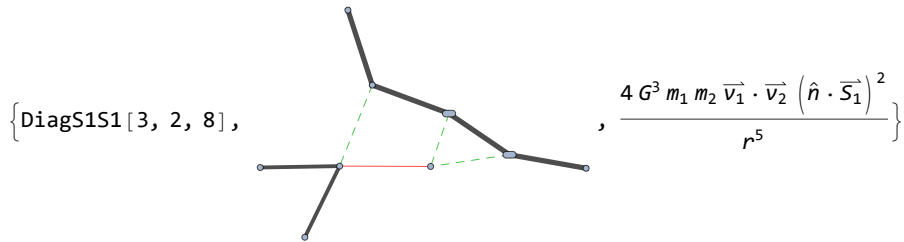
 $, \frac{4 G^3 m_1 m_2 \vec{v}_1 \cdot \vec{v}_2 (\hat{n} \cdot \vec{S}_1)^2}{r^5} \}$

$\{\text{DiagS1S1}[3, 2, 9],$ 
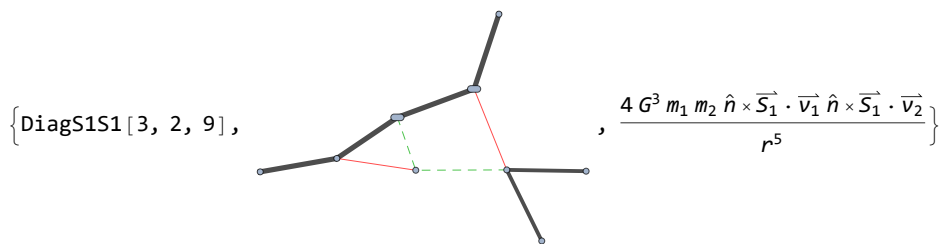
 $, \frac{4 G^3 m_1 m_2 \hat{n} \times \vec{S}_1 \cdot \vec{v}_1 \hat{n} \times \vec{S}_1 \cdot \vec{v}_2}{r^5} \}$

$\{\text{DiagS1S1}[3, 2, 10],$ 
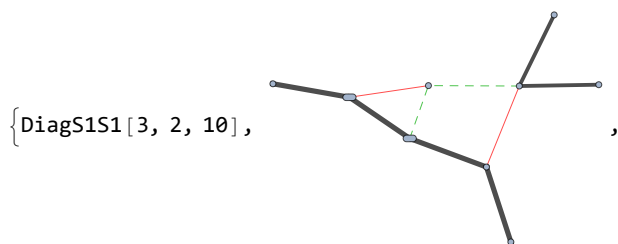
 $,$

$$\frac{G^3 m_1 m_2 \left( -8 \vec{S}_1 \cdot \vec{S}_1 \hat{n} \cdot \vec{v}_1 \hat{n} \cdot \vec{v}_2 + 8 \hat{n} \cdot \vec{S}_1 \hat{n} \cdot \vec{v}_2 \vec{S}_1 \cdot \vec{v}_1 + 4 \vec{S}_1 \cdot \vec{S}_1 \vec{v}_1 \cdot \vec{v}_2 - 4 \vec{S}_1 \cdot \vec{v}_1 \vec{S}_1 \cdot \vec{v}_2 \right)}{r^5} \}$$

$$\left\{ \text{DiagS1S1}[3, 2, 11], \frac{G^3 m_1 m_2 \left( \hat{n} \times \vec{S}_1 \cdot \vec{v}_1 \right)^2}{r^5} \right\}$$
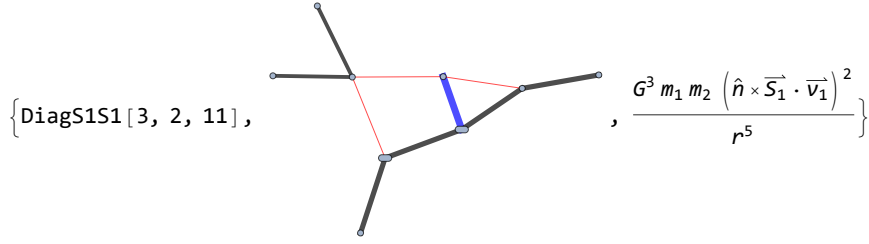

$$\left\{ \text{DiagS1S1}[3, 2, 12], \right.$$
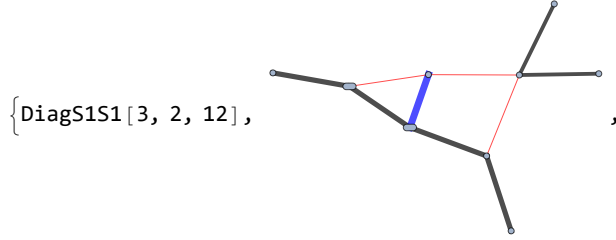

$$\frac{G^3 m_1 m_2 \left( 2 \left( \hat{n} \times \vec{S}_1 \cdot \vec{v}_1 \right)^2 - 6 \vec{S}_1 \cdot \vec{S}_1 \left( \hat{n} \cdot \vec{v}_1 \right)^2 + 6 \hat{n} \cdot \vec{S}_1 \hat{n} \cdot \vec{v}_1 \vec{S}_1 \cdot \vec{v}_1 - \left( \vec{S}_1 \cdot \vec{v}_1 \right)^2 + \vec{S}_1 \cdot \vec{S}_1 \vec{v}_1 \cdot \vec{v}_1 \right)}{r^5} \left. \right\}$$

$$\left\{ \text{DiagS1S1}[3, 2, 13], - \frac{G^3 m_1 m_2 \hat{n} \times \vec{S}_1 \cdot \vec{v}_1 \hat{n} \times \vec{S}_1 \cdot \vec{v}_2}{r^5} \right\}$$
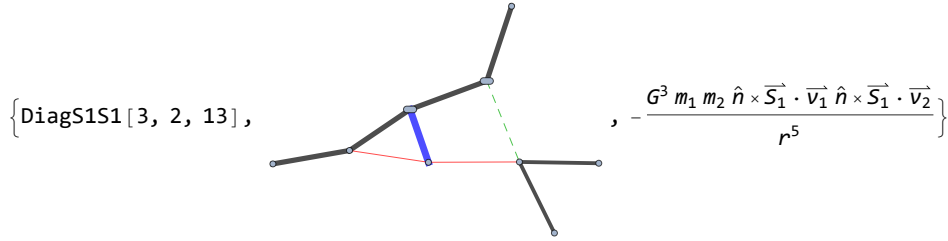

$$\left\{ \text{DiagS1S1}[3, 2, 14], - \frac{G^3 m_1 m_2 \left( \hat{n} \times \vec{S}_1 \cdot \vec{v}_1 \right)^2}{r^5} \right\}$$
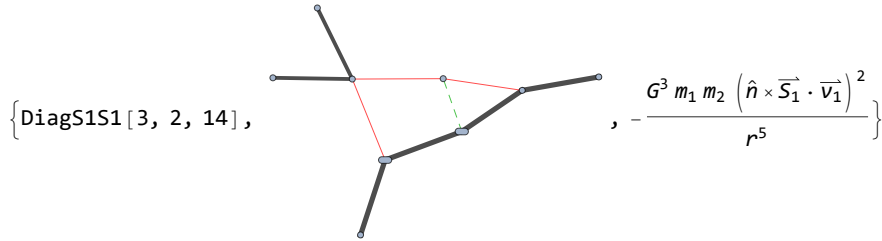

$$\left\{ \text{DiagS1S1}[3, 2, 15], \right.$$
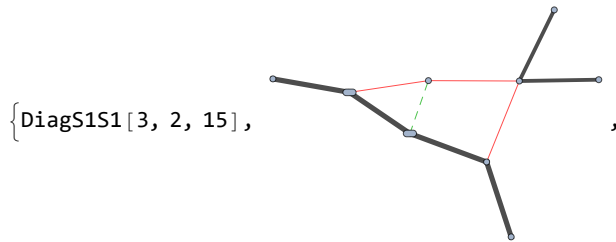

$$G^3 m_1 m_2 \left( \frac{\vec{S}_1 \cdot \vec{a}_1 \hat{n} \cdot \vec{S}_1 - \vec{S}_1 \cdot \vec{S}_1 \hat{n} \cdot \vec{a}_1 + \vec{S}_1 \cdot \vec{S}_1 \left( - \left( \hat{n} \cdot \vec{v}_1 \right) \right) + \hat{n} \cdot \vec{S}_1 \vec{S}_1 \cdot \vec{v}_1}{r^4} + \frac{1}{r^5} \left( -2 \left( \hat{n} \times \vec{S}_1 \cdot \vec{v}_1 \right)^2 + \vec{S}_1 \cdot \vec{S}_1 \left( \hat{n} \cdot \vec{v}_1 \right)^2 + \right. \right. \\ \left. \left. 5 \vec{S}_1 \cdot \vec{S}_1 \hat{n} \cdot \vec{v}_1 \hat{n} \cdot \vec{v}_2 - \hat{n} \cdot \vec{S}_1 \hat{n} \cdot \vec{v}_1 \vec{S}_1 \cdot \vec{v}_1 - 5 \hat{n} \cdot \vec{S}_1 \hat{n} \cdot \vec{v}_2 \vec{S}_1 \cdot \vec{v}_1 + \vec{S}_1 \cdot \vec{v}_1 \vec{S}_1 \cdot \vec{v}_2 - \vec{S}_1 \cdot \vec{S}_1 \vec{v}_1 \cdot \vec{v}_2 \right) \right) \left. \right\}$$

{DiagS1S1[3, 2, 16],

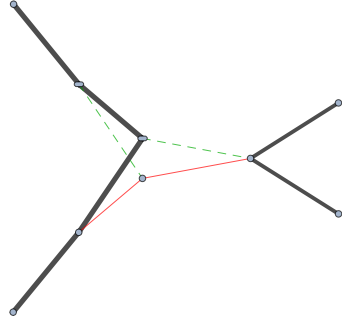

$$, \frac{G^3 m_1 m_2 \hat{n} \times \vec{S}_1 \cdot \vec{v}_1 \hat{n} \times \vec{S}_1 \cdot \vec{v}_2}{r^5} \}$$

{DiagS1S1[3, 2, 17],

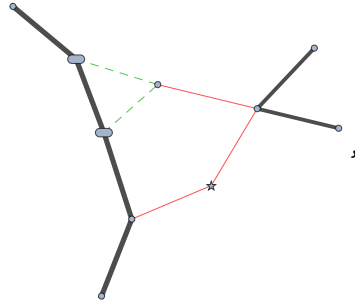

$$G^3 m_1 m_2 \left( \frac{-3 \left( \hat{n} \cdot \vec{S}_1 \right)^2 \left( \hat{n} \cdot \vec{v}_1 \right)^2 + \frac{7}{2} \left( \hat{n} \cdot \vec{S}_1 \right)^2 \hat{n} \cdot \vec{v}_1 \hat{n} \cdot \vec{v}_2 - \frac{1}{2} \vec{v}_1 \cdot \vec{v}_2 \left( \hat{n} \cdot \vec{S}_1 \right)^2 + \hat{n} \cdot \vec{S}_1 \hat{n} \cdot \vec{v}_1 \vec{S}_1 \cdot \vec{v}_1 - \hat{n} \cdot \vec{S}_1 \hat{n} \cdot \vec{v}_1 \vec{S}_1 \cdot \vec{v}_2}{r^5} + \frac{\hat{n} \cdot \vec{S}_1 \hat{n} \cdot \vec{S}_1 \hat{n} \cdot \vec{v}_1}{r^4} \right) \}$$

{DiagS1S1[3, 2, 18],

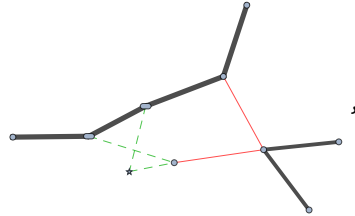

$$G^3 m_1 m_2 \left( \frac{1}{r^5} \left( 2 \left( \hat{n} \times \vec{S}_1 \cdot \vec{v}_1 \right)^2 + \frac{35}{4} \left( \hat{n} \cdot \vec{S}_1 \right)^2 \left( \hat{n} \cdot \vec{v}_1 \right)^2 - 14 \left( \hat{n} \cdot \vec{S}_1 \right)^2 \hat{n} \cdot \vec{v}_1 \hat{n} \cdot \vec{v}_2 + \frac{1}{4} \vec{S}_1 \cdot \vec{S}_1 \left( \hat{n} \cdot \vec{v}_1 \right)^2 + \right. \right. \\ \left. \frac{5}{2} \vec{S}_1 \cdot \vec{S}_1 \hat{n} \cdot \vec{v}_1 \hat{n} \cdot \vec{v}_2 - \frac{17}{2} \hat{n} \cdot \vec{S}_1 \hat{n} \cdot \vec{v}_1 \vec{S}_1 \cdot \vec{v}_1 + \frac{15}{2} \hat{n} \cdot \vec{S}_1 \hat{n} \cdot \vec{v}_2 \vec{S}_1 \cdot \vec{v}_1 + 4 \hat{n} \cdot \vec{S}_1 \hat{n} \cdot \vec{v}_1 \vec{S}_1 \cdot \vec{v}_2 - \right. \\ \left. \frac{5}{4} \vec{v}_1 \cdot \vec{v}_1 \left( \hat{n} \cdot \vec{S}_1 \right)^2 + 2 \vec{v}_1 \cdot \vec{v}_2 \left( \hat{n} \cdot \vec{S}_1 \right)^2 + 2 \left( \vec{S}_1 \cdot \vec{v}_1 \right)^2 - \frac{3}{2} \vec{S}_1 \cdot \vec{v}_1 \vec{S}_1 \cdot \vec{v}_2 - \frac{5}{4} \vec{S}_1 \cdot \vec{S}_1 \vec{v}_1 \cdot \vec{v}_1 - \frac{1}{2} \vec{S}_1 \cdot \vec{S}_1 \vec{v}_1 \cdot \vec{v}_2 \right) + \\ \left. \frac{1}{r^4} \left( -\frac{25}{2} \hat{n} \cdot \vec{S}_1 \hat{n} \cdot \vec{S}_1 \hat{n} \cdot \vec{v}_1 + \frac{9}{2} \vec{S}_1 \cdot \vec{S}_1 \hat{n} \cdot \vec{v}_1 + \frac{25}{2} \hat{n} \cdot \vec{S}_1 \hat{n} \cdot \vec{S}_1 \hat{n} \cdot \vec{v}_2 + 4 \hat{n} \cdot \vec{S}_1 \vec{S}_1 \cdot \vec{v}_1 - \frac{5}{2} \hat{n} \cdot \vec{S}_1 \vec{S}_1 \cdot \vec{v}_2 - \right. \right. \\ \left. \left. \frac{9}{2} \vec{S}_1 \cdot \vec{S}_1 \hat{n} \cdot \vec{v}_2 + \hat{n} \cdot \vec{S}_1 \vec{S}_1 \cdot \vec{v}_1 - \frac{5}{2} \hat{n} \cdot \vec{S}_1 \vec{S}_1 \cdot \vec{v}_2 \right) + \frac{\frac{5}{2} \left( \hat{n} \cdot \vec{S}_1 \right)^2 - \frac{3}{2} \vec{S}_1 \cdot \vec{S}_1}{r^3} \right) \}$$

{DiagS1S1[3, 2, 19],

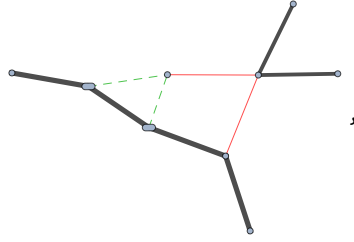

$$G^3 m_1 m_2 \left( \frac{2 \vec{S}_1 \cdot \vec{a}_1 \hat{n} \cdot \vec{S}_1 - 2 \vec{S}_1 \cdot \vec{S}_1 \hat{n} \cdot \vec{a}_1 - 2 \vec{S}_1 \cdot \vec{S}_1 \hat{n} \cdot \vec{v}_1 + 2 \hat{n} \cdot \vec{S}_1 \vec{S}_1 \cdot \vec{v}_1}{r^4} + \frac{1}{r^5} \left( - \left( \hat{n} \times \vec{S}_1 \cdot \vec{v}_1 \right)^2 + 3 \vec{S}_1 \cdot \vec{S}_1 \left( \hat{n} \cdot \vec{v}_1 \right)^2 - \right. \right.$$

$$\left. \left. 3 \hat{n} \cdot \vec{S}_1 \hat{n} \cdot \vec{v}_1 \vec{S}_1 \cdot \vec{v}_1 - \frac{3}{2} \vec{v}_1 \cdot \vec{v}_1 \left( \hat{n} \cdot \vec{S}_1 \right)^2 + \frac{9}{2} \vec{v}_2 \cdot \vec{v}_2 \left( \hat{n} \cdot \vec{S}_1 \right)^2 + \left( \vec{S}_1 \cdot \vec{v}_1 \right)^2 - \vec{S}_1 \cdot \vec{S}_1 \vec{v}_1 \cdot \vec{v}_1 \right) \right) \Bigg\}$$

{DiagS1S1[3, 3, 1],

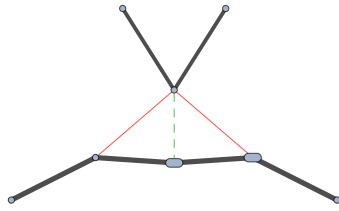

$$, - \frac{4 G^3 m_1 m_2 \hat{n} \times \vec{S}_1 \cdot \vec{v}_1 \hat{n} \times \vec{S}_1 \cdot \vec{v}_2}{r^5} \Bigg\}$$

{DiagS1S1[3, 3, 2],

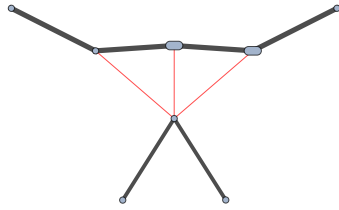

$$, \frac{2 G^3 m_1 m_2 \left( \hat{n} \times \vec{S}_1 \cdot \vec{v}_1 \right)^2}{r^5} \Bigg\}$$

{DiagS1S1[3, 4, 1],

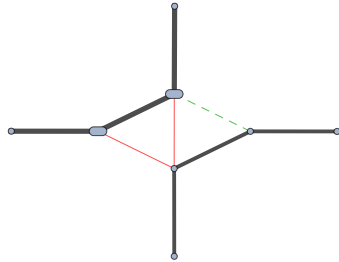

$$, - \frac{16 G^3 m_2^2 \hat{n} \times \vec{S}_1 \cdot \vec{v}_1 \hat{n} \times \vec{S}_1 \cdot \vec{v}_2}{r^5} \Bigg\}$$

{DiagS1S1[3, 4, 2],

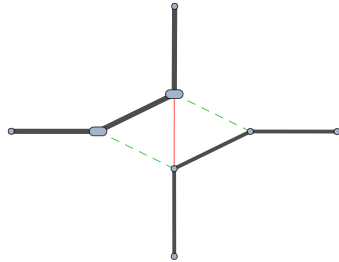

$$, \frac{16 G^3 m_2^2 \left( \hat{n} \times \vec{S}_1 \cdot \vec{v}_2 \right)^2}{r^5} \Bigg\}$$

{DiagS1S1[3, 4, 3],

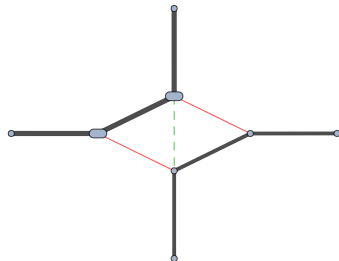

$$, - \frac{16 G^3 m_2^2 \hat{n} \times \vec{S}_1 \cdot \vec{v}_1 \hat{n} \times \vec{S}_1 \cdot \vec{v}_2}{r^5} \Bigg\}$$

{DiagS1S1[3, 5, 1],

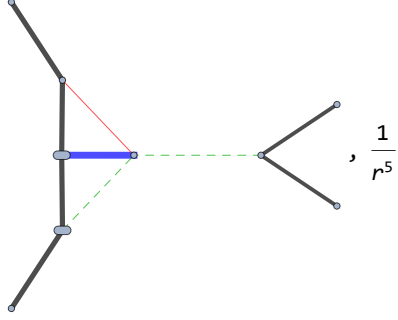

$$G^3 m_1 m_2 \left( -\frac{8}{7} \hat{n} \times \vec{S}_1 \cdot \vec{v}_1 \hat{n} \times \vec{S}_1 \cdot \vec{v}_2 + \frac{16}{7} \vec{v}_1 \cdot \vec{v}_2 (\hat{n} \cdot \vec{S}_1)^2 - \frac{72}{7} \hat{n} \cdot \vec{S}_1 \hat{n} \cdot \vec{v}_2 \vec{S}_1 \cdot \vec{v}_1 - \right. \\ \left. \frac{64}{7} \hat{n} \cdot \vec{S}_1 \hat{n} \cdot \vec{v}_1 \vec{S}_1 \cdot \vec{v}_2 + \frac{136}{7} \vec{S}_1 \cdot \vec{S}_1 \hat{n} \cdot \vec{v}_1 \hat{n} \cdot \vec{v}_2 + \frac{176}{35} \vec{S}_1 \cdot \vec{v}_1 \vec{S}_1 \cdot \vec{v}_2 - \frac{128}{35} \vec{S}_1 \cdot \vec{S}_1 \vec{v}_1 \cdot \vec{v}_2 \right) \Bigg\}$$

{DiagS1S1[3, 5, 2],

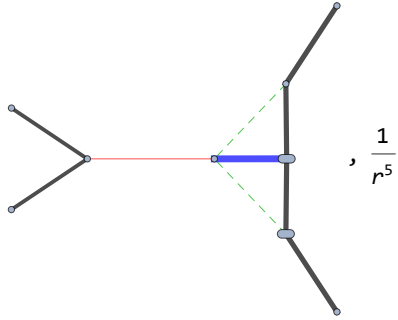

$$G^3 m_1 m_2 \left( \frac{8}{7} (\hat{n} \times \vec{S}_1 \cdot \vec{v}_1)^2 - \frac{16}{7} \vec{S}_1 \cdot \vec{S}_1 (\hat{n} \cdot \vec{v}_1)^2 + \frac{16}{7} \hat{n} \cdot \vec{S}_1 \hat{n} \cdot \vec{v}_1 \vec{S}_1 \cdot \vec{v}_1 + \right. \\ \left. \frac{8}{7} \vec{v}_1 \cdot \vec{v}_1 (\hat{n} \cdot \vec{S}_1)^2 - \frac{4}{35} (\vec{S}_1 \cdot \vec{v}_1)^2 - \frac{4}{5} \vec{S}_1 \cdot \vec{S}_1 \vec{v}_1 \cdot \vec{v}_1 \right) \Bigg\}$$

{DiagS1S1[3, 5, 3],

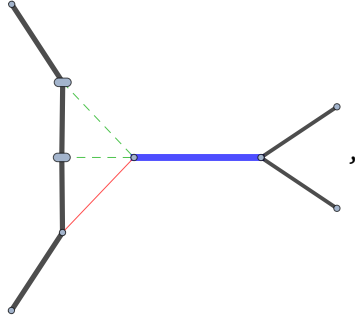

$$G^3 m_1 m_2 \left( \frac{1}{r^5 \in_d} \left( 4 (\hat{n} \cdot \vec{S}_1)^2 (\hat{n} \cdot \vec{v}_2)^2 - \frac{4}{7} \vec{v}_2 \cdot \vec{v}_2 (\hat{n} \cdot \vec{S}_1)^2 - \frac{16}{7} \hat{n} \cdot \vec{S}_1 \hat{n} \cdot \vec{v}_2 \vec{S}_1 \cdot \vec{v}_2 - \frac{4}{7} \vec{S}_1 \cdot \vec{S}_1 (\hat{n} \cdot \vec{v}_2)^2 + \right. \right. \\ \left. \frac{8}{35} (\vec{S}_1 \cdot \vec{v}_2)^2 + \frac{4}{35} \vec{S}_1 \cdot \vec{S}_1 \vec{v}_2 \cdot \vec{v}_2 \right) + \frac{1}{r^5} \log \left( \frac{r}{R_\theta} \right) \left( -12 (\hat{n} \cdot \vec{S}_1)^2 (\hat{n} \cdot \vec{v}_2)^2 + \frac{12}{7} \vec{v}_2 \cdot \vec{v}_2 (\hat{n} \cdot \vec{S}_1)^2 + \right. \\ \left. \frac{48}{7} \hat{n} \cdot \vec{S}_1 \hat{n} \cdot \vec{v}_2 \vec{S}_1 \cdot \vec{v}_2 + \frac{12}{7} \vec{S}_1 \cdot \vec{S}_1 (\hat{n} \cdot \vec{v}_2)^2 - \frac{24}{35} (\vec{S}_1 \cdot \vec{v}_2)^2 - \frac{12}{35} \vec{S}_1 \cdot \vec{S}_1 \vec{v}_2 \cdot \vec{v}_2 \right) + \frac{1}{r^5} \\ \left( \frac{12}{7} (\hat{n} \times \vec{S}_1 \cdot \vec{v}_2)^2 + \frac{28}{3} (\hat{n} \cdot \vec{S}_1)^2 (\hat{n} \cdot \vec{v}_2)^2 + \frac{92}{147} \vec{S}_1 \cdot \vec{S}_1 (\hat{n} \cdot \vec{v}_2)^2 - \frac{1312}{147} \hat{n} \cdot \vec{S}_1 \hat{n} \cdot \vec{v}_2 \vec{S}_1 \cdot \vec{v}_2 + \right. \\ \left. \frac{176}{147} \vec{v}_2 \cdot \vec{v}_2 (\hat{n} \cdot \vec{S}_1)^2 + \frac{8866}{3675} (\vec{S}_1 \cdot \vec{v}_2)^2 - \frac{5962}{3675} \vec{S}_1 \cdot \vec{S}_1 \vec{v}_2 \cdot \vec{v}_2 \right) \Bigg\}$$

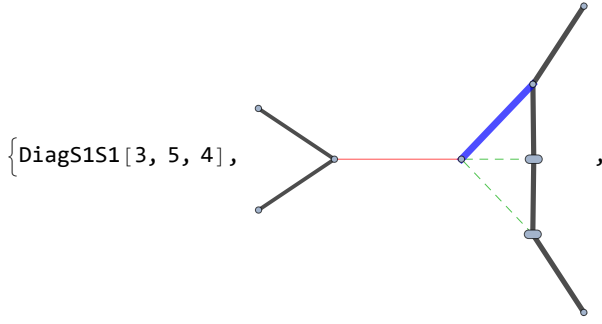

$$G^3 m_1 m_2 \left( \frac{1}{r^5 \in_d} \left( 4 \left( \hat{n} \cdot \vec{S}_1 \right)^2 \left( \hat{n} \cdot \vec{v}_1 \right)^2 - \frac{4}{7} \vec{v}_1 \cdot \vec{v}_1 \left( \hat{n} \cdot \vec{S}_1 \right)^2 - \frac{16}{7} \hat{n} \cdot \vec{S}_1 \hat{n} \cdot \vec{v}_1 \vec{S}_1 \cdot \vec{v}_1 - \frac{4}{7} \vec{S}_1 \cdot \vec{S}_1 \left( \hat{n} \cdot \vec{v}_1 \right)^2 + \right. \right. \\ \left. \frac{8}{35} \left( \vec{S}_1 \cdot \vec{v}_1 \right)^2 + \frac{4}{35} \vec{S}_1 \cdot \vec{S}_1 \vec{v}_1 \cdot \vec{v}_1 \right) + \frac{1}{r^5} \log \left( \frac{r}{R_\theta} \right) \left( -12 \left( \hat{n} \cdot \vec{S}_1 \right)^2 \left( \hat{n} \cdot \vec{v}_1 \right)^2 + \frac{12}{7} \vec{v}_1 \cdot \vec{v}_1 \left( \hat{n} \cdot \vec{S}_1 \right)^2 + \right. \\ \left. \frac{48}{7} \hat{n} \cdot \vec{S}_1 \hat{n} \cdot \vec{v}_1 \vec{S}_1 \cdot \vec{v}_1 + \frac{12}{7} \vec{S}_1 \cdot \vec{S}_1 \left( \hat{n} \cdot \vec{v}_1 \right)^2 - \frac{24}{35} \left( \vec{S}_1 \cdot \vec{v}_1 \right)^2 - \frac{12}{35} \vec{S}_1 \cdot \vec{S}_1 \vec{v}_1 \cdot \vec{v}_1 \right) + \frac{1}{r^5} \\ \left( \frac{12}{7} \left( \hat{n} \times \vec{S}_1 \cdot \vec{v}_1 \right)^2 + \frac{28}{3} \left( \hat{n} \cdot \vec{S}_1 \right)^2 \left( \hat{n} \cdot \vec{v}_1 \right)^2 + \frac{92}{147} \vec{S}_1 \cdot \vec{S}_1 \left( \hat{n} \cdot \vec{v}_1 \right)^2 - \frac{1312}{147} \hat{n} \cdot \vec{S}_1 \hat{n} \cdot \vec{v}_1 \vec{S}_1 \cdot \vec{v}_1 + \right. \\ \left. \frac{176}{147} \vec{v}_1 \cdot \vec{v}_1 \left( \hat{n} \cdot \vec{S}_1 \right)^2 + \frac{8866 \left( \vec{S}_1 \cdot \vec{v}_1 \right)^2}{3675} - \frac{5962 \vec{S}_1 \cdot \vec{S}_1 \vec{v}_1 \cdot \vec{v}_1}{3675} \right) \Bigg\}$$

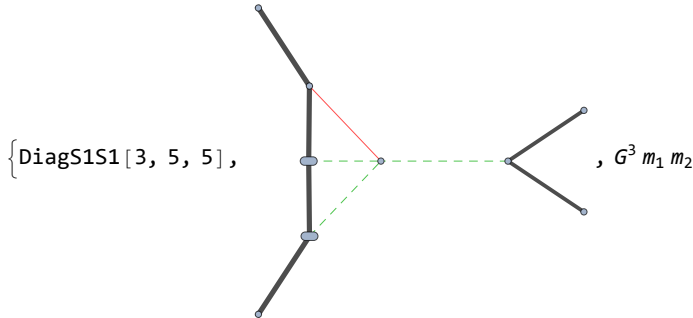

$$\left( \frac{-\frac{320}{49} \hat{n} \cdot \vec{a}_2 \left( \hat{n} \cdot \vec{S}_1 \right)^2 - \frac{464}{49} \hat{n} \cdot \vec{S}_1 \hat{n} \cdot \vec{v}_2 \hat{n} \cdot \vec{S}_1 + \frac{528 \vec{S}_1 \cdot \vec{v}_2 \hat{n} \cdot \vec{S}_1}{1225} + \frac{4432 \vec{S}_1 \cdot \vec{a}_2 \hat{n} \cdot \vec{S}_1}{1225} + \frac{9488 \hat{n} \cdot \vec{v}_2 \vec{S}_1 \cdot \vec{S}_1}{1225} + \frac{3056 \hat{n} \cdot \vec{a}_2 \vec{S}_1 \cdot \vec{S}_1}{1225} + \frac{528 \hat{n} \cdot \vec{S}_1 \vec{S}_1 \cdot \vec{v}_2}{1225}}{r^4} \right. \\ \left. + \frac{1}{r^5} \left( -56 \left( \hat{n} \cdot \vec{v}_2 \right)^2 \left( \hat{n} \cdot \vec{S}_1 \right)^2 + \frac{112}{3} \hat{n} \cdot \vec{v}_1 \hat{n} \cdot \vec{v}_2 \left( \hat{n} \cdot \vec{S}_1 \right)^2 - \frac{808}{147} \vec{v}_1 \cdot \vec{v}_2 \left( \hat{n} \cdot \vec{S}_1 \right)^2 + \right. \right. \\ \frac{320}{49} \vec{v}_2 \cdot \vec{v}_2 \left( \hat{n} \cdot \vec{S}_1 \right)^2 - \frac{1280}{147} \hat{n} \cdot \vec{v}_2 \vec{S}_1 \cdot \vec{v}_1 \hat{n} \cdot \vec{S}_1 - \frac{608}{147} \hat{n} \cdot \vec{v}_1 \vec{S}_1 \cdot \vec{v}_2 \hat{n} \cdot \vec{S}_1 + \\ \frac{1728}{49} \hat{n} \cdot \vec{v}_2 \vec{S}_1 \cdot \vec{v}_2 \hat{n} \cdot \vec{S}_1 - \frac{4432 \left( \vec{S}_1 \cdot \vec{v}_2 \right)^2}{1225} + \frac{32}{7} \hat{n} \times \vec{S}_1 \cdot \vec{v}_1 \hat{n} \times \vec{S}_1 \cdot \vec{v}_2 + \frac{712}{49} \left( \hat{n} \cdot \vec{v}_2 \right)^2 \vec{S}_1 \cdot \vec{S}_1 - \\ \left. \frac{2992}{147} \hat{n} \cdot \vec{v}_1 \hat{n} \cdot \vec{v}_2 \vec{S}_1 \cdot \vec{S}_1 + \frac{2704 \vec{S}_1 \cdot \vec{v}_1 \vec{S}_1 \cdot \vec{v}_2}{3675} + \frac{15632 \vec{S}_1 \cdot \vec{S}_1 \vec{v}_1 \cdot \vec{v}_2}{3675} - \frac{3056 \vec{S}_1 \cdot \vec{S}_1 \vec{v}_2 \cdot \vec{v}_2}{1225} \right) + \\ \left( \frac{1}{r^4} \left( \frac{72}{7} \hat{n} \cdot \vec{a}_2 \left( \hat{n} \cdot \vec{S}_1 \right)^2 + \frac{96}{7} \hat{n} \cdot \vec{S}_1 \hat{n} \cdot \vec{v}_2 \hat{n} \cdot \vec{S}_1 - \frac{96}{35} \vec{S}_1 \cdot \vec{v}_2 \hat{n} \cdot \vec{S}_1 - \frac{144}{35} \vec{S}_1 \cdot \vec{a}_2 \hat{n} \cdot \vec{S}_1 - \right. \right.$$

$$\begin{aligned}
& \left( \frac{96}{35} \hat{n} \cdot \vec{v}_2 \vec{S}_1 \cdot \vec{S}_1 - \frac{72}{35} \hat{n} \cdot \vec{a}_2 \vec{S}_1 \cdot \vec{S}_1 - \frac{96}{35} \hat{n} \cdot \vec{S}_1 \vec{S}_1 \cdot \vec{v}_2 \right) + \frac{1}{r^5} \\
& \left( 72 (\hat{n} \cdot \vec{v}_2)^2 (\hat{n} \cdot \vec{S}_1)^2 - 48 \hat{n} \cdot \vec{v}_1 \hat{n} \cdot \vec{v}_2 (\hat{n} \cdot \vec{S}_1)^2 + \frac{48}{7} \vec{v}_1 \cdot \vec{v}_2 (\hat{n} \cdot \vec{S}_1)^2 - \frac{72}{7} \vec{v}_2 \cdot \vec{v}_2 (\hat{n} \cdot \vec{S}_1)^2 + \right. \\
& \frac{96}{7} \hat{n} \cdot \vec{v}_2 \vec{S}_1 \cdot \vec{v}_1 \hat{n} \cdot \vec{S}_1 + \frac{96}{7} \hat{n} \cdot \vec{v}_1 \vec{S}_1 \cdot \vec{v}_2 \hat{n} \cdot \vec{S}_1 - \frac{288}{7} \hat{n} \cdot \vec{v}_2 \vec{S}_1 \cdot \vec{v}_2 \hat{n} \cdot \vec{S}_1 + \frac{144}{35} (\vec{S}_1 \cdot \vec{v}_2)^2 - \\
& \left. \frac{72}{7} (\hat{n} \cdot \vec{v}_2)^2 \vec{S}_1 \cdot \vec{S}_1 + \frac{48}{7} \hat{n} \cdot \vec{v}_1 \hat{n} \cdot \vec{v}_2 \vec{S}_1 \cdot \vec{S}_1 - \frac{96}{35} \vec{S}_1 \cdot \vec{v}_1 \vec{S}_1 \cdot \vec{v}_2 - \frac{48}{35} \vec{S}_1 \cdot \vec{S}_1 \vec{v}_1 \cdot \vec{v}_2 + \frac{72}{35} \vec{S}_1 \cdot \vec{S}_1 \vec{v}_2 \cdot \vec{v}_2 \right) \\
& \log \left( \frac{r}{R_\theta} \right) + \frac{1}{\epsilon_d} \left( \frac{1}{r^4} \left( -\frac{24}{7} \hat{n} \cdot \vec{a}_2 (\hat{n} \cdot \vec{S}_1)^2 - \frac{32}{7} \hat{n} \cdot \vec{S}_1 \hat{n} \cdot \vec{v}_2 \hat{n} \cdot \vec{S}_1 + \frac{32}{35} \vec{S}_1 \cdot \vec{v}_2 \hat{n} \cdot \vec{S}_1 + \right. \right. \\
& \left. \frac{48}{35} \vec{S}_1 \cdot \vec{a}_2 \hat{n} \cdot \vec{S}_1 + \frac{32}{35} \hat{n} \cdot \vec{v}_2 \vec{S}_1 \cdot \vec{S}_1 + \frac{24}{35} \hat{n} \cdot \vec{a}_2 \vec{S}_1 \cdot \vec{S}_1 + \frac{32}{35} \hat{n} \cdot \vec{S}_1 \vec{S}_1 \cdot \vec{v}_2 \right) + \frac{1}{r^5} \\
& \left( -24 (\hat{n} \cdot \vec{v}_2)^2 (\hat{n} \cdot \vec{S}_1)^2 + 16 \hat{n} \cdot \vec{v}_1 \hat{n} \cdot \vec{v}_2 (\hat{n} \cdot \vec{S}_1)^2 - \frac{16}{7} \vec{v}_1 \cdot \vec{v}_2 (\hat{n} \cdot \vec{S}_1)^2 + \frac{24}{7} \vec{v}_2 \cdot \vec{v}_2 (\hat{n} \cdot \vec{S}_1)^2 - \right. \\
& \left. \frac{32}{7} \hat{n} \cdot \vec{v}_2 \vec{S}_1 \cdot \vec{v}_1 \hat{n} \cdot \vec{S}_1 - \frac{32}{7} \hat{n} \cdot \vec{v}_1 \vec{S}_1 \cdot \vec{v}_2 \hat{n} \cdot \vec{S}_1 + \frac{96}{7} \hat{n} \cdot \vec{v}_2 \vec{S}_1 \cdot \vec{v}_2 \hat{n} \cdot \vec{S}_1 - \frac{48}{35} (\vec{S}_1 \cdot \vec{v}_2)^2 + \right. \\
& \left. \frac{24}{7} (\hat{n} \cdot \vec{v}_2)^2 \vec{S}_1 \cdot \vec{S}_1 - \frac{16}{7} \hat{n} \cdot \vec{v}_1 \hat{n} \cdot \vec{v}_2 \vec{S}_1 \cdot \vec{S}_1 + \frac{32}{35} \vec{S}_1 \cdot \vec{v}_1 \vec{S}_1 \cdot \vec{v}_2 + \frac{16}{35} \vec{S}_1 \cdot \vec{S}_1 \vec{v}_1 \cdot \vec{v}_2 - \frac{24}{35} \vec{S}_1 \cdot \vec{S}_1 \vec{v}_2 \cdot \vec{v}_2 \right) \Bigg) \Bigg\}
\end{aligned}$$

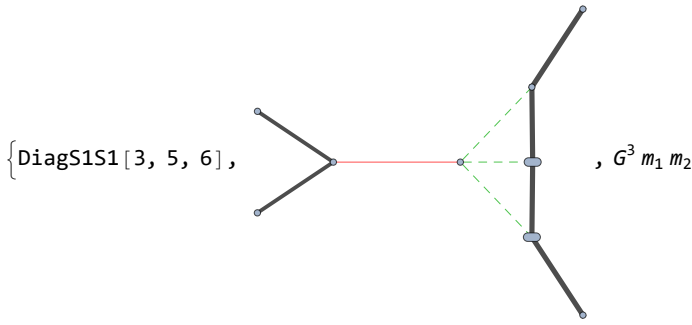

$$\begin{aligned}
& \left( -\frac{320}{49} \hat{n} \cdot \vec{a}_1 (\hat{n} \cdot \vec{S}_1)^2 + \frac{464}{49} \hat{n} \cdot \vec{S}_1 \hat{n} \cdot \vec{v}_1 \hat{n} \cdot \vec{S}_1 - \frac{4448 \vec{S}_1 \cdot \vec{v}_1 \hat{n} \cdot \vec{S}_1}{1225} + \frac{4432 \vec{S}_1 \cdot \vec{a}_1 \hat{n} \cdot \vec{S}_1}{1225} - \frac{5568 \hat{n} \cdot \vec{v}_1 \vec{S}_1 \cdot \vec{S}_1}{1225} + \frac{3056 \hat{n} \cdot \vec{a}_1 \vec{S}_1 \cdot \vec{S}_1}{1225} - \frac{528 \hat{n} \cdot \vec{S}_1 \vec{S}_1 \cdot \vec{v}_1}{1225} \right) \\
& \frac{1}{r^4} \\
& + \frac{1}{r^5} \left( -\frac{32}{7} (\hat{n} \cdot \vec{S}_1 \cdot \vec{v}_1)^2 - \frac{56}{3} (\hat{n} \cdot \vec{S}_1)^2 (\hat{n} \cdot \vec{v}_1)^2 - \frac{10592 (\vec{S}_1 \cdot \vec{v}_1)^2}{3675} + \right. \\
& \left. \frac{488}{147} (\hat{n} \cdot \vec{v}_1)^2 \vec{S}_1 \cdot \vec{S}_1 + \frac{1952}{147} \hat{n} \cdot \vec{S}_1 \hat{n} \cdot \vec{v}_1 \vec{S}_1 \cdot \vec{v}_1 + \frac{152}{147} (\hat{n} \cdot \vec{S}_1)^2 \vec{v}_1 \cdot \vec{v}_1 + \frac{6464 \vec{S}_1 \cdot \vec{S}_1 \vec{v}_1 \cdot \vec{v}_1}{3675} \right) + \\
& \left( \frac{1}{r^4} \left( \frac{72}{7} \hat{n} \cdot \vec{a}_1 (\hat{n} \cdot \vec{S}_1)^2 - \frac{96}{7} \hat{n} \cdot \vec{S}_1 \hat{n} \cdot \vec{v}_1 \hat{n} \cdot \vec{S}_1 + \frac{96}{35} \vec{S}_1 \cdot \vec{v}_1 \hat{n} \cdot \vec{S}_1 - \frac{144}{35} \vec{S}_1 \cdot \vec{a}_1 \hat{n} \cdot \vec{S}_1 + \frac{96}{35} \hat{n} \cdot \vec{v}_1 \vec{S}_1 \cdot \vec{S}_1 - \right. \right. \\
& \left. \frac{72}{35} \hat{n} \cdot \vec{a}_1 \vec{S}_1 \cdot \vec{S}_1 + \frac{96}{35} \hat{n} \cdot \vec{S}_1 \vec{S}_1 \cdot \vec{v}_1 \right) + \frac{1}{r^5} \left( 24 (\hat{n} \cdot \vec{v}_1)^2 (\hat{n} \cdot \vec{S}_1)^2 - \frac{24}{7} \vec{v}_1 \cdot \vec{v}_1 (\hat{n} \cdot \vec{S}_1)^2 - \right. \\
& \left. \frac{96}{7} \hat{n} \cdot \vec{v}_1 \vec{S}_1 \cdot \vec{v}_1 \hat{n} \cdot \vec{S}_1 + \frac{48}{35} (\vec{S}_1 \cdot \vec{v}_1)^2 - \frac{24}{7} (\hat{n} \cdot \vec{v}_1)^2 \vec{S}_1 \cdot \vec{S}_1 + \frac{24}{35} \vec{S}_1 \cdot \vec{S}_1 \vec{v}_1 \cdot \vec{v}_1 \right) \Bigg) \log \left( \frac{r}{R_\theta} \right) + \frac{1}{\epsilon_d} \\
& \left( \frac{1}{r^4} \left( -\frac{24}{7} \hat{n} \cdot \vec{a}_1 (\hat{n} \cdot \vec{S}_1)^2 + \frac{32}{7} \hat{n} \cdot \vec{S}_1 \hat{n} \cdot \vec{v}_1 \hat{n} \cdot \vec{S}_1 - \frac{32}{35} \vec{S}_1 \cdot \vec{v}_1 \hat{n} \cdot \vec{S}_1 + \frac{48}{35} \vec{S}_1 \cdot \vec{a}_1 \hat{n} \cdot \vec{S}_1 - \frac{32}{35} \hat{n} \cdot \vec{v}_1 \vec{S}_1 \cdot \vec{S}_1 + \right. \right. \\
& \left. \frac{24}{35} \hat{n} \cdot \vec{a}_1 \vec{S}_1 \cdot \vec{S}_1 - \frac{32}{35} \hat{n} \cdot \vec{S}_1 \vec{S}_1 \cdot \vec{v}_1 \right) + \frac{1}{r^5} \left( -8 (\hat{n} \cdot \vec{v}_1)^2 (\hat{n} \cdot \vec{S}_1)^2 + \frac{8}{7} \vec{v}_1 \cdot \vec{v}_1 (\hat{n} \cdot \vec{S}_1)^2 + \right.
\end{aligned}$$

$$\left. \left. \frac{32}{7} \hat{n} \cdot \vec{v}_1 \vec{S}_1 \cdot \vec{v}_1 \hat{n} \cdot \vec{S}_1 - \frac{16}{35} \left( \vec{S}_1 \cdot \vec{v}_1 \right)^2 + \frac{8}{7} \left( \hat{n} \cdot \vec{v}_1 \right)^2 \vec{S}_1 \cdot \vec{S}_1 - \frac{8}{35} \vec{S}_1 \cdot \vec{S}_1 \vec{v}_1 \cdot \vec{v}_1 \right) \right) \right\}$$

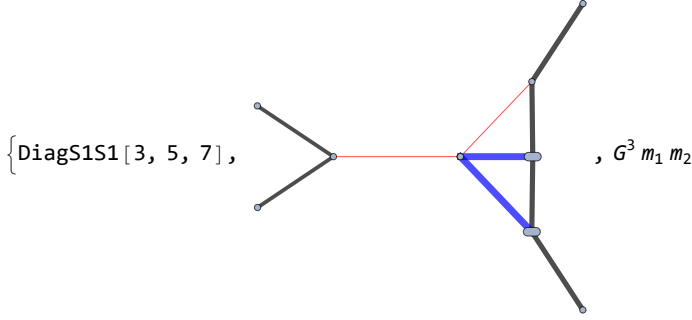

$$\left( \frac{2 \left( \hat{n} \cdot \vec{S}_1 \right)^2 \left( \hat{n} \cdot \vec{v}_1 \right)^2 - \frac{2}{7} \vec{v}_1 \cdot \vec{v}_1 \left( \hat{n} \cdot \vec{S}_1 \right)^2 - \frac{8}{7} \hat{n} \cdot \vec{S}_1 \hat{n} \cdot \vec{v}_1 \vec{S}_1 \cdot \vec{v}_1 - \frac{2}{7} \vec{S}_1 \cdot \vec{S}_1 \left( \hat{n} \cdot \vec{v}_1 \right)^2 + \frac{4}{35} \left( \vec{S}_1 \cdot \vec{v}_1 \right)^2 + \frac{2}{35} \vec{S}_1 \cdot \vec{S}_1 \vec{v}_1 \cdot \vec{v}_1}{r^5 \in_d} \right. \\ + \frac{1}{r^5} \log \left( \frac{r}{R_0} \right) \left( -6 \left( \hat{n} \cdot \vec{S}_1 \right)^2 \left( \hat{n} \cdot \vec{v}_1 \right)^2 + \frac{6}{7} \vec{v}_1 \cdot \vec{v}_1 \left( \hat{n} \cdot \vec{S}_1 \right)^2 + \right. \\ \left. \frac{24}{7} \hat{n} \cdot \vec{S}_1 \hat{n} \cdot \vec{v}_1 \vec{S}_1 \cdot \vec{v}_1 + \frac{6}{7} \vec{S}_1 \cdot \vec{S}_1 \left( \hat{n} \cdot \vec{v}_1 \right)^2 - \frac{12}{35} \left( \vec{S}_1 \cdot \vec{v}_1 \right)^2 - \frac{6}{35} \vec{S}_1 \cdot \vec{S}_1 \vec{v}_1 \cdot \vec{v}_1 \right) + \\ \left. \frac{1}{r^5} \left( -\frac{6}{7} \left( \hat{n} \times \vec{S}_1 \cdot \vec{v}_1 \right)^2 + 7 \left( \hat{n} \cdot \vec{S}_1 \right)^2 \left( \hat{n} \cdot \vec{v}_1 \right)^2 - \frac{127}{49} \vec{S}_1 \cdot \vec{S}_1 \left( \hat{n} \cdot \vec{v}_1 \right)^2 - \frac{158}{49} \hat{n} \cdot \vec{S}_1 \hat{n} \cdot \vec{v}_1 \vec{S}_1 \cdot \vec{v}_1 - \right. \right. \\ \left. \left. \frac{71}{49} \vec{v}_1 \cdot \vec{v}_1 \left( \hat{n} \cdot \vec{S}_1 \right)^2 + \frac{136 \left( \vec{S}_1 \cdot \vec{v}_1 \right)^2}{1225} + \frac{1293 \vec{S}_1 \cdot \vec{S}_1 \vec{v}_1 \cdot \vec{v}_1}{1225} \right) \right) \right\}$$

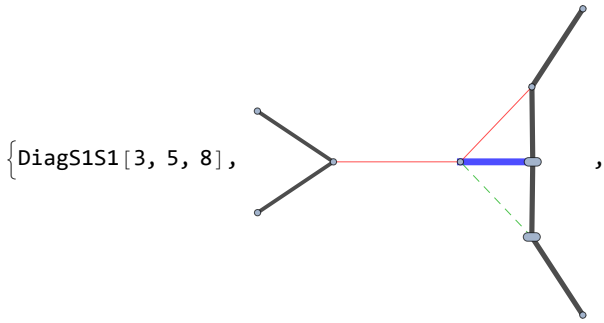

$$G^3 m_1 m_2 \left( \frac{1}{r^5} \left( -\frac{2}{7} \left( \hat{n} \times \vec{S}_1 \cdot \vec{v}_1 \right)^2 - 7 \left( \hat{n} \cdot \vec{S}_1 \right)^2 \left( \hat{n} \cdot \vec{v}_1 \right)^2 - \frac{206 \left( \vec{S}_1 \cdot \vec{v}_1 \right)^2}{1225} - 7 \left( \hat{n} \cdot \vec{S}_1 \right)^2 \hat{n} \cdot \vec{v}_1 \hat{n} \cdot \vec{v}_2 + \frac{155}{49} \left( \hat{n} \cdot \vec{v}_1 \right)^2 \vec{S}_1 \cdot \vec{S}_1 + \right. \right. \\ \left. \frac{141}{49} \hat{n} \cdot \vec{v}_1 \hat{n} \cdot \vec{v}_2 \vec{S}_1 \cdot \vec{S}_1 + \frac{130}{49} \hat{n} \cdot \vec{S}_1 \hat{n} \cdot \vec{v}_1 \vec{S}_1 \cdot \vec{v}_1 + \frac{58}{49} \hat{n} \cdot \vec{S}_1 \hat{n} \cdot \vec{v}_2 \vec{S}_1 \cdot \vec{v}_1 + \frac{86}{49} \hat{n} \cdot \vec{S}_1 \hat{n} \cdot \vec{v}_1 \vec{S}_1 \cdot \vec{v}_2 - \right. \\ \left. \frac{206 \vec{S}_1 \cdot \vec{v}_1 \vec{S}_1 \cdot \vec{v}_2}{1225} + \frac{43}{49} \left( \hat{n} \cdot \vec{S}_1 \right)^2 \vec{v}_1 \cdot \vec{v}_1 - \frac{663 \vec{S}_1 \cdot \vec{S}_1 \vec{v}_1 \cdot \vec{v}_1}{1225} + \frac{43}{49} \left( \hat{n} \cdot \vec{S}_1 \right)^2 \vec{v}_1 \cdot \vec{v}_2 - \frac{663 \vec{S}_1 \cdot \vec{S}_1 \vec{v}_1 \cdot \vec{v}_2}{1225} \right) + \\ \left. \frac{1}{r^5} \left( 6 \left( \hat{n} \cdot \vec{v}_1 \right)^2 \left( \hat{n} \cdot \vec{S}_1 \right)^2 + 6 \hat{n} \cdot \vec{v}_1 \hat{n} \cdot \vec{v}_2 \left( \hat{n} \cdot \vec{S}_1 \right)^2 - \frac{6}{7} \vec{v}_1 \cdot \vec{v}_1 \left( \hat{n} \cdot \vec{S}_1 \right)^2 - \frac{6}{7} \vec{v}_1 \cdot \vec{v}_2 \left( \hat{n} \cdot \vec{S}_1 \right)^2 - \right. \right. \\ \left. \frac{24}{7} \hat{n} \cdot \vec{v}_1 \vec{S}_1 \cdot \vec{v}_1 \hat{n} \cdot \vec{S}_1 - \frac{12}{7} \hat{n} \cdot \vec{v}_2 \vec{S}_1 \cdot \vec{v}_1 \hat{n} \cdot \vec{S}_1 - \frac{12}{7} \hat{n} \cdot \vec{v}_1 \vec{S}_1 \cdot \vec{v}_2 \hat{n} \cdot \vec{S}_1 + \frac{12}{35} \left( \vec{S}_1 \cdot \vec{v}_1 \right)^2 - \frac{6}{7} \left( \hat{n} \cdot \vec{v}_1 \right)^2 \vec{S}_1 \cdot \vec{S}_1 - \right. \\ \left. \frac{6}{7} \hat{n} \cdot \vec{v}_1 \hat{n} \cdot \vec{v}_2 \vec{S}_1 \cdot \vec{S}_1 + \frac{12}{35} \vec{S}_1 \cdot \vec{v}_1 \vec{S}_1 \cdot \vec{v}_2 + \frac{6}{35} \vec{S}_1 \cdot \vec{S}_1 \vec{v}_1 \cdot \vec{v}_1 + \frac{6}{35} \vec{S}_1 \cdot \vec{S}_1 \vec{v}_1 \cdot \vec{v}_2 \right) \log \left( \frac{r}{R_0} \right) +$$

$$\frac{1}{r^5 \in_d} \left( -2 (\hat{n} \cdot \vec{v}_1)^2 (\hat{n} \cdot \vec{S}_1)^2 - 2 \hat{n} \cdot \vec{v}_1 \hat{n} \cdot \vec{v}_2 (\hat{n} \cdot \vec{S}_1)^2 + \frac{2}{7} \vec{v}_1 \cdot \vec{v}_1 (\hat{n} \cdot \vec{S}_1)^2 + \frac{2}{7} \vec{v}_1 \cdot \vec{v}_2 (\hat{n} \cdot \vec{S}_1)^2 + \right. \\ \left. \frac{8}{7} \hat{n} \cdot \vec{v}_1 \vec{S}_1 \cdot \vec{v}_1 \hat{n} \cdot \vec{S}_1 + \frac{4}{7} \hat{n} \cdot \vec{v}_2 \vec{S}_1 \cdot \vec{v}_1 \hat{n} \cdot \vec{S}_1 + \frac{4}{7} \hat{n} \cdot \vec{v}_1 \vec{S}_1 \cdot \vec{v}_2 \hat{n} \cdot \vec{S}_1 - \frac{4}{35} (\vec{S}_1 \cdot \vec{v}_1)^2 + \right. \\ \left. \frac{2}{7} (\hat{n} \cdot \vec{v}_1)^2 \vec{S}_1 \cdot \vec{S}_1 + \frac{2}{7} \hat{n} \cdot \vec{v}_1 \hat{n} \cdot \vec{v}_2 \vec{S}_1 \cdot \vec{S}_1 - \frac{4}{35} \vec{S}_1 \cdot \vec{v}_1 \vec{S}_1 \cdot \vec{v}_2 - \frac{2}{35} \vec{S}_1 \cdot \vec{S}_1 \vec{v}_1 \cdot \vec{v}_1 - \frac{2}{35} \vec{S}_1 \cdot \vec{S}_1 \vec{v}_1 \cdot \vec{v}_2 \right) \Bigg\}$$

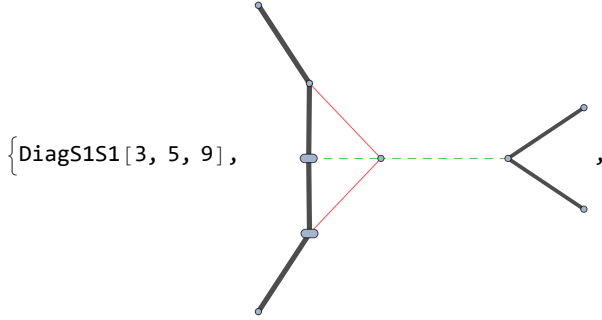

$$\frac{G^3 m_1 m_2 \left( \frac{32}{7} \hat{n} \times \vec{S}_1 \cdot \vec{v}_1 \hat{n} \times \vec{S}_1 \cdot \vec{v}_2 - \frac{96}{7} \vec{S}_1 \cdot \vec{S}_1 \hat{n} \cdot \vec{v}_1 \hat{n} \cdot \vec{v}_2 + \frac{96}{7} \hat{n} \cdot \vec{S}_1 \hat{n} \cdot \vec{v}_2 \vec{S}_1 \cdot \vec{v}_1 - \frac{256}{35} \vec{S}_1 \cdot \vec{v}_1 \vec{S}_1 \cdot \vec{v}_2 + \frac{256}{35} \vec{S}_1 \cdot \vec{S}_1 \vec{v}_1 \cdot \vec{v}_2 \right)}{r^5} \Bigg\}$$

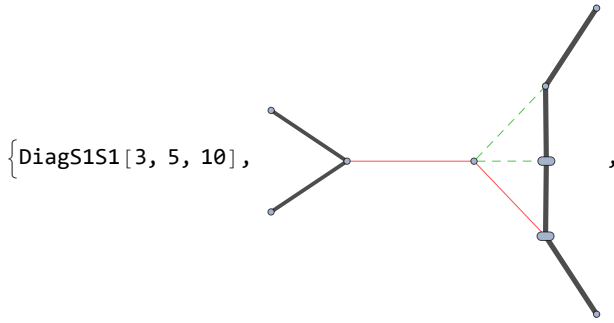

$$\frac{G^3 m_1 m_2 \left( -\frac{32}{7} (\hat{n} \times \vec{S}_1 \cdot \vec{v}_1)^2 - \frac{16}{35} (\vec{S}_1 \cdot \vec{v}_1)^2 + \frac{16}{35} \vec{S}_1 \cdot \vec{S}_1 \vec{v}_1 \cdot \vec{v}_1 \right)}{r^5} \Bigg\}$$

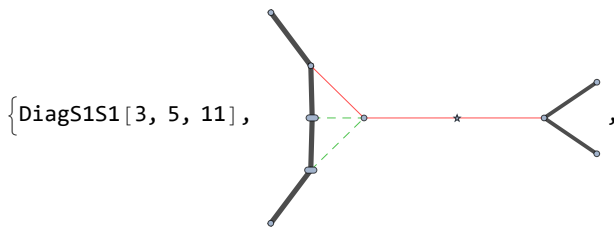

$$G^3 m_1 m_2 \left( \frac{-\frac{8}{49} \hat{n} \cdot \vec{S}_1 \hat{n} \cdot \vec{S}_1 \hat{n} \cdot \vec{v}_2 + \frac{572 \vec{S}_1 \cdot \vec{S}_1 \hat{n} \cdot \vec{v}_2}{1225} + \frac{292 \hat{n} \cdot \vec{S}_1 \vec{S}_1 \cdot \vec{v}_2}{1225} + \frac{292 \hat{n} \cdot \vec{S}_1 \vec{S}_1 \cdot \vec{v}_2}{1225}}{r^4} + \right. \\ \left. \frac{1}{r^5} \left( -2 \hat{n} \cdot \vec{v}_1 \hat{n} \cdot \vec{v}_2 (\hat{n} \cdot \vec{S}_1)^2 - \frac{4}{49} \vec{v}_1 \cdot \vec{v}_2 (\hat{n} \cdot \vec{S}_1)^2 - \frac{8}{49} \hat{n} \cdot \vec{v}_2 \vec{S}_1 \cdot \vec{v}_1 \hat{n} \cdot \vec{S}_1 - \right. \right. \\ \left. \left. \frac{8}{49} \hat{n} \cdot \vec{v}_1 \vec{S}_1 \cdot \vec{v}_2 \hat{n} \cdot \vec{S}_1 - \frac{32}{49} \hat{n} \cdot \vec{v}_1 \hat{n} \cdot \vec{v}_2 \vec{S}_1 \cdot \vec{S}_1 + \frac{292 \vec{S}_1 \cdot \vec{v}_1 \vec{S}_1 \cdot \vec{v}_2}{1225} + \frac{286 \vec{S}_1 \cdot \vec{S}_1 \vec{v}_1 \cdot \vec{v}_2}{1225} \right) \right) +$$

$$\left( \frac{-\frac{36}{7} \hat{n} \cdot \vec{S}_1 \hat{n} \cdot \vec{S}_1 \hat{n} \cdot \vec{v}_2 + \frac{36}{35} \vec{S}_1 \cdot \vec{S}_1 \hat{n} \cdot \vec{v}_2 + \frac{36}{35} \hat{n} \cdot \vec{S}_1 \vec{S}_1 \cdot \vec{v}_2 + \frac{36}{35} \hat{n} \cdot \vec{S}_1 \vec{S}_1 \cdot \vec{v}_2}{r^4} + \frac{1}{r^5} \right. \\ \left. \left( 18 \hat{n} \cdot \vec{v}_1 \hat{n} \cdot \vec{v}_2 \left( \hat{n} \cdot \vec{S}_1 \right)^2 - \frac{18}{7} \vec{v}_1 \cdot \vec{v}_2 \left( \hat{n} \cdot \vec{S}_1 \right)^2 - \frac{36}{7} \hat{n} \cdot \vec{v}_2 \vec{S}_1 \cdot \vec{v}_1 \hat{n} \cdot \vec{S}_1 - \frac{36}{7} \hat{n} \cdot \vec{v}_1 \vec{S}_1 \cdot \vec{v}_2 \hat{n} \cdot \vec{S}_1 - \right. \right. \\ \left. \left. \frac{18}{7} \hat{n} \cdot \vec{v}_1 \hat{n} \cdot \vec{v}_2 \vec{S}_1 \cdot \vec{S}_1 + \frac{36}{35} \vec{S}_1 \cdot \vec{v}_1 \vec{S}_1 \cdot \vec{v}_2 + \frac{18}{35} \vec{S}_1 \cdot \vec{S}_1 \vec{v}_1 \cdot \vec{v}_2 \right) \log \left( \frac{r}{R_\theta} \right) + \right. \\ \left. \frac{1}{\epsilon_d} \left( \frac{\frac{12}{7} \hat{n} \cdot \vec{S}_1 \hat{n} \cdot \vec{S}_1 \hat{n} \cdot \vec{v}_2 - \frac{12}{35} \vec{S}_1 \cdot \vec{S}_1 \hat{n} \cdot \vec{v}_2 - \frac{12}{35} \hat{n} \cdot \vec{S}_1 \vec{S}_1 \cdot \vec{v}_2 - \frac{12}{35} \hat{n} \cdot \vec{S}_1 \vec{S}_1 \cdot \vec{v}_2}{r^4} + \frac{1}{r^5} \right. \right. \\ \left. \left. \left( -6 \hat{n} \cdot \vec{v}_1 \hat{n} \cdot \vec{v}_2 \left( \hat{n} \cdot \vec{S}_1 \right)^2 + \frac{6}{7} \vec{v}_1 \cdot \vec{v}_2 \left( \hat{n} \cdot \vec{S}_1 \right)^2 + \frac{12}{7} \hat{n} \cdot \vec{v}_2 \vec{S}_1 \cdot \vec{v}_1 \hat{n} \cdot \vec{S}_1 + \right. \right. \\ \left. \left. \frac{12}{7} \hat{n} \cdot \vec{v}_1 \vec{S}_1 \cdot \vec{v}_2 \hat{n} \cdot \vec{S}_1 + \frac{6}{7} \hat{n} \cdot \vec{v}_1 \hat{n} \cdot \vec{v}_2 \vec{S}_1 \cdot \vec{S}_1 - \frac{12}{35} \vec{S}_1 \cdot \vec{v}_1 \vec{S}_1 \cdot \vec{v}_2 - \frac{6}{35} \vec{S}_1 \cdot \vec{S}_1 \vec{v}_1 \cdot \vec{v}_2 \right) \right) \right) \Bigg\}$$

{DiagS1S1[3, 5, 12],

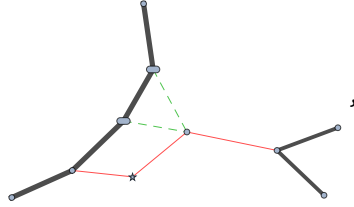

$$G^3 m_1 m_2 \left( \frac{\frac{76}{49} \hat{n} \cdot \vec{S}_1 \hat{n} \cdot \vec{S}_1 \hat{n} \cdot \vec{v}_1 + \frac{852 \vec{S}_1 \cdot \vec{S}_1 \hat{n} \cdot \vec{v}_1}{1225} + \frac{292 \hat{n} \cdot \vec{S}_1 \vec{S}_1 \cdot \vec{v}_1}{1225} + \frac{292 \hat{n} \cdot \vec{S}_1 \vec{S}_1 \cdot \vec{v}_1}{1225}}{r^4} + \frac{1}{r^5} \right. \\ \left( -\frac{20}{3} \left( \hat{n} \cdot \vec{v}_1 \right)^2 \left( \hat{n} \cdot \vec{S}_1 \right)^2 + 8 \hat{n} \cdot \vec{v}_1 \hat{n} \cdot \vec{v}_2 \left( \hat{n} \cdot \vec{S}_1 \right)^2 - \frac{20}{147} \vec{v}_1 \cdot \vec{v}_1 \left( \hat{n} \cdot \vec{S}_1 \right)^2 - \frac{38}{49} \vec{v}_1 \cdot \vec{v}_2 \left( \hat{n} \cdot \vec{S}_1 \right)^2 + \right. \\ \left. \frac{172}{147} \hat{n} \cdot \vec{v}_1 \vec{S}_1 \cdot \vec{v}_1 \hat{n} \cdot \vec{S}_1 + \frac{8}{49} \hat{n} \cdot \vec{v}_2 \vec{S}_1 \cdot \vec{v}_1 \hat{n} \cdot \vec{S}_1 - \frac{76}{49} \hat{n} \cdot \vec{v}_1 \vec{S}_1 \cdot \vec{v}_2 \hat{n} \cdot \vec{S}_1 + \frac{802 \left( \vec{S}_1 \cdot \vec{v}_1 \right)^2}{3675} - \right. \\ \left. \frac{160}{147} \left( \hat{n} \cdot \vec{v}_1 \right)^2 \vec{S}_1 \cdot \vec{S}_1 + \frac{60}{49} \hat{n} \cdot \vec{v}_1 \hat{n} \cdot \vec{v}_2 \vec{S}_1 \cdot \vec{S}_1 - \frac{292 \vec{S}_1 \cdot \vec{v}_1 \vec{S}_1 \cdot \vec{v}_2}{1225} + \frac{262 \vec{S}_1 \cdot \vec{S}_1 \vec{v}_1 \cdot \vec{v}_1}{1225} - \frac{426 \vec{S}_1 \cdot \vec{S}_1 \vec{v}_1 \cdot \vec{v}_2}{1225} \right) + \\ \left( -\frac{36}{7} \hat{n} \cdot \vec{S}_1 \hat{n} \cdot \vec{S}_1 \hat{n} \cdot \vec{v}_1 + \frac{36}{35} \vec{S}_1 \cdot \vec{S}_1 \hat{n} \cdot \vec{v}_1 + \frac{36}{35} \hat{n} \cdot \vec{S}_1 \vec{S}_1 \cdot \vec{v}_1 + \frac{36}{35} \hat{n} \cdot \vec{S}_1 \vec{S}_1 \cdot \vec{v}_1}{r^4} + \frac{1}{r^5} \right. \\ \left( 16 \left( \hat{n} \cdot \vec{v}_1 \right)^2 \left( \hat{n} \cdot \vec{S}_1 \right)^2 - 18 \hat{n} \cdot \vec{v}_1 \hat{n} \cdot \vec{v}_2 \left( \hat{n} \cdot \vec{S}_1 \right)^2 - \frac{16}{7} \vec{v}_1 \cdot \vec{v}_1 \left( \hat{n} \cdot \vec{S}_1 \right)^2 + \frac{18}{7} \vec{v}_1 \cdot \vec{v}_2 \left( \hat{n} \cdot \vec{S}_1 \right)^2 - \right. \\ \left. \frac{64}{7} \hat{n} \cdot \vec{v}_1 \vec{S}_1 \cdot \vec{v}_1 \hat{n} \cdot \vec{S}_1 + \frac{36}{7} \hat{n} \cdot \vec{v}_2 \vec{S}_1 \cdot \vec{v}_1 \hat{n} \cdot \vec{S}_1 + \frac{36}{7} \hat{n} \cdot \vec{v}_1 \vec{S}_1 \cdot \vec{v}_2 \hat{n} \cdot \vec{S}_1 + \frac{32}{35} \left( \vec{S}_1 \cdot \vec{v}_1 \right)^2 - \frac{16}{7} \left( \hat{n} \cdot \vec{v}_1 \right)^2 \vec{S}_1 \cdot \vec{S}_1 + \right. \\ \left. \frac{18}{7} \hat{n} \cdot \vec{v}_1 \hat{n} \cdot \vec{v}_2 \vec{S}_1 \cdot \vec{S}_1 - \frac{36}{35} \vec{S}_1 \cdot \vec{v}_1 \vec{S}_1 \cdot \vec{v}_2 + \frac{16}{35} \vec{S}_1 \cdot \vec{S}_1 \vec{v}_1 \cdot \vec{v}_1 - \frac{18}{35} \vec{S}_1 \cdot \vec{S}_1 \vec{v}_1 \cdot \vec{v}_2 \right) \log \left( \frac{r}{R_\theta} \right) + \right. \\ \left. \left. \left. \right. \right. \right)$$

$$\frac{1}{\epsilon_d} \left( \frac{\frac{12}{7} \hat{n} \cdot \vec{S}_1 \hat{n} \cdot \vec{S}_1 \hat{n} \cdot \vec{v}_1 - \frac{12}{35} \vec{S}_1 \cdot \vec{S}_1 \hat{n} \cdot \vec{v}_1 - \frac{12}{35} \hat{n} \cdot \vec{S}_1 \vec{S}_1 \cdot \vec{v}_1 - \frac{12}{35} \hat{n} \cdot \vec{S}_1 \vec{S}_1 \cdot \vec{v}_1}{r^4} + \frac{1}{r^5} \right. \\ \left. \left( -\frac{16}{3} (\hat{n} \cdot \vec{v}_1)^2 (\hat{n} \cdot \vec{S}_1)^2 + 6 \hat{n} \cdot \vec{v}_1 \hat{n} \cdot \vec{v}_2 (\hat{n} \cdot \vec{S}_1)^2 + \frac{16}{21} \vec{v}_1 \cdot \vec{v}_1 (\hat{n} \cdot \vec{S}_1)^2 - \frac{6}{7} \vec{v}_1 \cdot \vec{v}_2 (\hat{n} \cdot \vec{S}_1)^2 + \right. \right. \\ \left. \frac{64}{21} \hat{n} \cdot \vec{v}_1 \vec{S}_1 \cdot \vec{v}_1 \hat{n} \cdot \vec{S}_1 - \frac{12}{7} \hat{n} \cdot \vec{v}_2 \vec{S}_1 \cdot \vec{v}_1 \hat{n} \cdot \vec{S}_1 - \frac{12}{7} \hat{n} \cdot \vec{v}_1 \vec{S}_1 \cdot \vec{v}_2 \hat{n} \cdot \vec{S}_1 - \frac{32}{105} (\vec{S}_1 \cdot \vec{v}_1)^2 + \right. \\ \left. \left. \frac{16}{21} (\hat{n} \cdot \vec{v}_1)^2 \vec{S}_1 \cdot \vec{S}_1 - \frac{6}{7} \hat{n} \cdot \vec{v}_1 \hat{n} \cdot \vec{v}_2 \vec{S}_1 \cdot \vec{S}_1 + \frac{12}{35} \vec{S}_1 \cdot \vec{v}_1 \vec{S}_1 \cdot \vec{v}_2 - \frac{16}{105} \vec{S}_1 \cdot \vec{S}_1 \vec{v}_1 \cdot \vec{v}_1 + \frac{6}{35} \vec{S}_1 \cdot \vec{S}_1 \vec{v}_1 \cdot \vec{v}_2 \right) \right) \Bigg\}$$

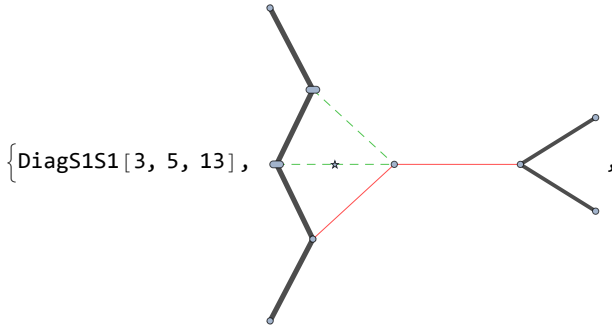

$$G^3 m_1 m_2 \left( \frac{\frac{8}{15} \vec{S}_1 \cdot \vec{S}_1 - \frac{8}{5} (\hat{n} \cdot \vec{S}_1)^2}{r^3} + \frac{1}{r^4} \left( 20 \hat{n} \cdot \vec{S}_1 \hat{n} \cdot \vec{S}_1 \hat{n} \cdot \vec{v}_1 - \frac{28}{5} \vec{S}_1 \cdot \vec{S}_1 \hat{n} \cdot \vec{v}_1 - 20 \hat{n} \cdot \vec{S}_1 \hat{n} \cdot \vec{S}_1 \hat{n} \cdot \vec{v}_2 + \right. \right. \\ \left. \frac{4}{5} \hat{n} \cdot \vec{S}_1 \vec{S}_1 \cdot \vec{v}_1 + \frac{8}{5} \hat{n} \cdot \vec{S}_1 \vec{S}_1 \cdot \vec{v}_2 + \frac{28}{5} \hat{n} \cdot \vec{v}_2 \vec{S}_1 \cdot \vec{S}_1 - 4 \hat{n} \cdot \vec{S}_1 \vec{S}_1 \cdot \vec{v}_1 + \frac{8}{5} \hat{n} \cdot \vec{S}_1 \vec{S}_1 \cdot \vec{v}_2 \right) + \frac{1}{r^5} \\ \left( \frac{24}{7} (\hat{n} \cdot \vec{S}_1 \cdot \vec{v}_1)^2 - 28 (\hat{n} \cdot \vec{S}_1)^2 (\hat{n} \cdot \vec{v}_1)^2 + \frac{2036 (\vec{S}_1 \cdot \vec{v}_1)^2}{1225} + 44 (\hat{n} \cdot \vec{S}_1)^2 \hat{n} \cdot \vec{v}_1 \hat{n} \cdot \vec{v}_2 + \frac{432}{49} (\hat{n} \cdot \vec{v}_1)^2 \vec{S}_1 \cdot \vec{S}_1 - \right. \\ \left. \frac{432}{49} \hat{n} \cdot \vec{v}_1 \hat{n} \cdot \vec{v}_2 \vec{S}_1 \cdot \vec{S}_1 + \frac{1180}{147} \hat{n} \cdot \vec{S}_1 \hat{n} \cdot \vec{v}_1 \vec{S}_1 \cdot \vec{v}_1 - \frac{332}{49} \hat{n} \cdot \vec{S}_1 \hat{n} \cdot \vec{v}_2 \vec{S}_1 \cdot \vec{v}_1 - \frac{472}{49} \hat{n} \cdot \vec{S}_1 \hat{n} \cdot \vec{v}_1 \vec{S}_1 \cdot \vec{v}_2 + \right. \\ \left. \frac{652 \vec{S}_1 \cdot \vec{v}_1 \vec{S}_1 \cdot \vec{v}_2}{1225} + \frac{400}{147} (\hat{n} \cdot \vec{S}_1)^2 \vec{v}_1 \cdot \vec{v}_1 - \frac{13396 \vec{S}_1 \cdot \vec{S}_1 \vec{v}_1 \cdot \vec{v}_1}{3675} - \frac{236}{49} (\hat{n} \cdot \vec{S}_1)^2 \vec{v}_1 \cdot \vec{v}_2 + \frac{1656 \vec{S}_1 \cdot \vec{S}_1 \vec{v}_1 \cdot \vec{v}_2}{1225} \right) + \\ \left( \frac{12 (\hat{n} \cdot \vec{S}_1)^2}{r^3} - 4 \vec{S}_1 \cdot \vec{S}_1 \right. \\ \left. \frac{1}{r^4} \left( -60 \hat{n} \cdot \vec{S}_1 \hat{n} \cdot \vec{S}_1 \hat{n} \cdot \vec{v}_1 + 12 \vec{S}_1 \cdot \vec{S}_1 \hat{n} \cdot \vec{v}_1 + 60 \hat{n} \cdot \vec{S}_1 \hat{n} \cdot \vec{S}_1 \hat{n} \cdot \vec{v}_2 + \right. \right. \\ \left. 12 \hat{n} \cdot \vec{S}_1 \vec{S}_1 \cdot \vec{v}_1 - 12 \hat{n} \cdot \vec{S}_1 \vec{S}_1 \cdot \vec{v}_2 - 12 \hat{n} \cdot \vec{v}_2 \vec{S}_1 \cdot \vec{S}_1 + 12 \hat{n} \cdot \vec{S}_1 \vec{S}_1 \cdot \vec{v}_1 - 12 \hat{n} \cdot \vec{S}_1 \vec{S}_1 \cdot \vec{v}_2 \right) + \frac{1}{r^5} \\ \left( 44 (\hat{n} \cdot \vec{v}_1)^2 (\hat{n} \cdot \vec{S}_1)^2 - 72 \hat{n} \cdot \vec{v}_1 \hat{n} \cdot \vec{v}_2 (\hat{n} \cdot \vec{S}_1)^2 - \frac{44}{7} \vec{v}_1 \cdot \vec{v}_1 (\hat{n} \cdot \vec{S}_1)^2 + \frac{72}{7} \vec{v}_1 \cdot \vec{v}_2 (\hat{n} \cdot \vec{S}_1)^2 - \right. \\ \left. \frac{176}{7} \hat{n} \cdot \vec{v}_1 \vec{S}_1 \cdot \vec{v}_1 \hat{n} \cdot \vec{S}_1 + \frac{144}{7} \hat{n} \cdot \vec{v}_2 \vec{S}_1 \cdot \vec{v}_1 \hat{n} \cdot \vec{S}_1 + \frac{144}{7} \hat{n} \cdot \vec{v}_1 \vec{S}_1 \cdot \vec{v}_2 \hat{n} \cdot \vec{S}_1 + \frac{88}{35} (\vec{S}_1 \cdot \vec{v}_1)^2 - \frac{44}{7} (\hat{n} \cdot \vec{v}_1)^2 \right) \Bigg\}$$

$$\left. \begin{aligned} & \left( \vec{S}_1 \cdot \vec{S}_1 + \frac{72}{7} \hat{n} \cdot \vec{v}_1 \hat{n} \cdot \vec{v}_2 \vec{S}_1 \cdot \vec{S}_1 - \frac{144}{35} \vec{S}_1 \cdot \vec{v}_1 \vec{S}_1 \cdot \vec{v}_2 + \frac{44}{35} \vec{S}_1 \cdot \vec{S}_1 \vec{v}_1 \cdot \vec{v}_1 - \frac{72}{35} \vec{S}_1 \cdot \vec{S}_1 \vec{v}_1 \cdot \vec{v}_2 \right) \log \left( \frac{r}{R_\theta} \right) + \\ & \frac{1}{\epsilon_d} \left( \frac{\frac{4}{3} \vec{S}_1 \cdot \vec{S}_1 - 4 \left( \hat{n} \cdot \vec{S}_1 \right)^2}{r^3} + \frac{1}{r^4} \left( 20 \hat{n} \cdot \vec{S}_1 \hat{n} \cdot \vec{S}_1 \hat{n} \cdot \vec{v}_1 - 4 \vec{S}_1 \cdot \vec{S}_1 \hat{n} \cdot \vec{v}_1 - 20 \hat{n} \cdot \vec{S}_1 \hat{n} \cdot \vec{S}_1 \hat{n} \cdot \vec{v}_2 - \right. \right. \\ & \left. \left. 4 \hat{n} \cdot \vec{S}_1 \vec{S}_1 \cdot \vec{v}_1 + 4 \hat{n} \cdot \vec{S}_1 \vec{S}_1 \cdot \vec{v}_2 + 4 \hat{n} \cdot \vec{v}_2 \vec{S}_1 \cdot \vec{S}_1 - 4 \hat{n} \cdot \vec{S}_1 \vec{S}_1 \cdot \vec{v}_1 + 4 \hat{n} \cdot \vec{S}_1 \vec{S}_1 \cdot \vec{v}_2 \right) + \frac{1}{r^5} \right. \\ & \left( -\frac{44}{3} \left( \hat{n} \cdot \vec{v}_1 \right)^2 \left( \hat{n} \cdot \vec{S}_1 \right)^2 + 24 \hat{n} \cdot \vec{v}_1 \hat{n} \cdot \vec{v}_2 \left( \hat{n} \cdot \vec{S}_1 \right)^2 + \frac{44}{21} \vec{v}_1 \cdot \vec{v}_1 \left( \hat{n} \cdot \vec{S}_1 \right)^2 - \frac{24}{7} \vec{v}_1 \cdot \vec{v}_2 \left( \hat{n} \cdot \vec{S}_1 \right)^2 + \right. \\ & \left. \frac{176}{21} \hat{n} \cdot \vec{v}_1 \vec{S}_1 \cdot \vec{v}_1 \hat{n} \cdot \vec{S}_1 - \frac{48}{7} \hat{n} \cdot \vec{v}_2 \vec{S}_1 \cdot \vec{v}_1 \hat{n} \cdot \vec{S}_1 - \frac{48}{7} \hat{n} \cdot \vec{v}_1 \vec{S}_1 \cdot \vec{v}_2 \hat{n} \cdot \vec{S}_1 - \frac{88}{105} \left( \vec{S}_1 \cdot \vec{v}_1 \right)^2 + \right. \\ & \left. \left. \frac{44}{21} \left( \hat{n} \cdot \vec{v}_1 \right)^2 \vec{S}_1 \cdot \vec{S}_1 - \frac{24}{7} \hat{n} \cdot \vec{v}_1 \hat{n} \cdot \vec{v}_2 \vec{S}_1 \cdot \vec{S}_1 + \frac{48}{35} \vec{S}_1 \cdot \vec{v}_1 \vec{S}_1 \cdot \vec{v}_2 - \frac{44}{105} \vec{S}_1 \cdot \vec{S}_1 \vec{v}_1 \cdot \vec{v}_1 + \frac{24}{35} \vec{S}_1 \cdot \vec{S}_1 \vec{v}_1 \cdot \vec{v}_2 \right) \right) \right\} \end{aligned}$$

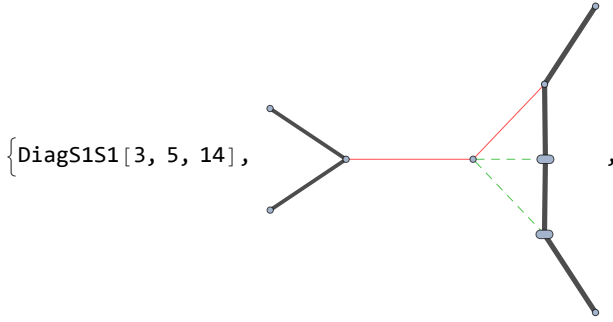

$$\begin{aligned} & G^3 m_1 m_2 \left( \frac{-\frac{16}{5} \hat{n} \cdot \vec{v}_1 \vec{S}_1 \cdot \vec{S}_1 + \frac{16}{5} \hat{n} \cdot \vec{S}_1 \vec{S}_1 \cdot \vec{a}_1 - \frac{16}{5} \hat{n} \cdot \vec{a}_1 \vec{S}_1 \cdot \vec{S}_1 + \frac{16}{5} \hat{n} \cdot \vec{S}_1 \vec{S}_1 \cdot \vec{v}_1}{r^4} + \frac{1}{r^5} \right. \\ & \left( -\frac{12}{7} \left( \hat{n} \cdot \vec{S}_1 \cdot \vec{v}_1 \right)^2 + \frac{68}{35} \left( \vec{S}_1 \cdot \vec{v}_1 \right)^2 + 7 \left( \hat{n} \cdot \vec{S}_1 \right)^2 \hat{n} \cdot \vec{v}_1 \hat{n} \cdot \vec{v}_2 + \frac{36}{7} \left( \hat{n} \cdot \vec{v}_1 \right)^2 \vec{S}_1 \cdot \vec{S}_1 - \frac{141}{49} \hat{n} \cdot \vec{v}_1 \hat{n} \cdot \vec{v}_2 \vec{S}_1 \cdot \vec{S}_1 - \right. \\ & \frac{36}{7} \hat{n} \cdot \vec{S}_1 \hat{n} \cdot \vec{v}_1 \vec{S}_1 \cdot \vec{v}_1 - \frac{58}{49} \hat{n} \cdot \vec{S}_1 \hat{n} \cdot \vec{v}_2 \vec{S}_1 \cdot \vec{v}_1 - \frac{86}{49} \hat{n} \cdot \vec{S}_1 \hat{n} \cdot \vec{v}_1 \vec{S}_1 \cdot \vec{v}_2 + \frac{206 \vec{S}_1 \cdot \vec{v}_1 \vec{S}_1 \cdot \vec{v}_2}{1225} - \frac{18}{7} \left( \hat{n} \cdot \vec{S}_1 \right)^2 \vec{v}_1 \cdot \vec{v}_1 - \\ & \left. \frac{16}{7} \vec{S}_1 \cdot \vec{S}_1 \vec{v}_1 \cdot \vec{v}_1 - \frac{43}{49} \left( \hat{n} \cdot \vec{S}_1 \right)^2 \vec{v}_1 \cdot \vec{v}_2 + \frac{663 \vec{S}_1 \cdot \vec{S}_1 \vec{v}_1 \cdot \vec{v}_2}{1225} - \frac{18}{7} \left( \hat{n} \cdot \vec{S}_1 \right)^2 \vec{v}_2 \cdot \vec{v}_2 - \frac{12}{35} \vec{S}_1 \cdot \vec{S}_1 \vec{v}_2 \cdot \vec{v}_2 \right) + \\ & \frac{1}{r^5} \left( -6 \hat{n} \cdot \vec{v}_1 \hat{n} \cdot \vec{v}_2 \left( \hat{n} \cdot \vec{S}_1 \right)^2 + \frac{6}{7} \vec{v}_1 \cdot \vec{v}_2 \left( \hat{n} \cdot \vec{S}_1 \right)^2 + \frac{12}{7} \hat{n} \cdot \vec{v}_2 \vec{S}_1 \cdot \vec{v}_1 \hat{n} \cdot \vec{S}_1 + \frac{12}{7} \hat{n} \cdot \vec{v}_1 \vec{S}_1 \cdot \vec{v}_2 \hat{n} \cdot \vec{S}_1 + \right. \\ & \left. \frac{6}{7} \hat{n} \cdot \vec{v}_1 \hat{n} \cdot \vec{v}_2 \vec{S}_1 \cdot \vec{S}_1 - \frac{12}{35} \vec{S}_1 \cdot \vec{v}_1 \vec{S}_1 \cdot \vec{v}_2 - \frac{6}{35} \vec{S}_1 \cdot \vec{S}_1 \vec{v}_1 \cdot \vec{v}_2 \right) \log \left( \frac{r}{R_\theta} \right) + \frac{1}{r^5 \epsilon_d} \\ & \left( 2 \hat{n} \cdot \vec{v}_1 \hat{n} \cdot \vec{v}_2 \left( \hat{n} \cdot \vec{S}_1 \right)^2 - \frac{2}{7} \vec{v}_1 \cdot \vec{v}_2 \left( \hat{n} \cdot \vec{S}_1 \right)^2 - \frac{4}{7} \hat{n} \cdot \vec{v}_2 \vec{S}_1 \cdot \vec{v}_1 \hat{n} \cdot \vec{S}_1 - \frac{4}{7} \hat{n} \cdot \vec{v}_1 \vec{S}_1 \cdot \vec{v}_2 \hat{n} \cdot \vec{S}_1 - \right. \\ & \left. \left. \frac{2}{7} \hat{n} \cdot \vec{v}_1 \hat{n} \cdot \vec{v}_2 \vec{S}_1 \cdot \vec{S}_1 + \frac{4}{35} \vec{S}_1 \cdot \vec{v}_1 \vec{S}_1 \cdot \vec{v}_2 + \frac{2}{35} \vec{S}_1 \cdot \vec{S}_1 \vec{v}_1 \cdot \vec{v}_2 \right) \right\} \end{aligned}$$

$\left\{ \text{DiagS1S1}[3, 6, 1], \right.$ 
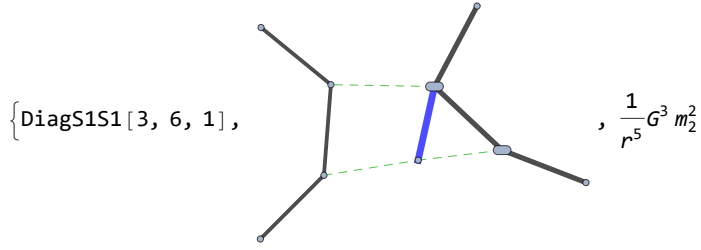
 $\left. , \frac{1}{r^5} G^3 m_2^2 \right\}$

$$\left\{ 22 \left( \hat{n} \times \vec{S}_1 \cdot \vec{v}_2 \right)^2 + 10 \vec{S}_1 \cdot \vec{S}_1 \left( \hat{n} \cdot \vec{v}_2 \right)^2 - 10 \hat{n} \cdot \vec{S}_1 \hat{n} \cdot \vec{v}_2 \vec{S}_1 \cdot \vec{v}_2 + 2 \vec{v}_2 \cdot \vec{v}_2 \left( \hat{n} \cdot \vec{S}_1 \right)^2 + 8 \left( \vec{S}_1 \cdot \vec{v}_2 \right)^2 - 10 \vec{S}_1 \cdot \vec{S}_1 \vec{v}_2 \cdot \vec{v}_2 \right\}$$

$\left\{ \text{DiagS1S1}[3, 6, 2], \right.$ 
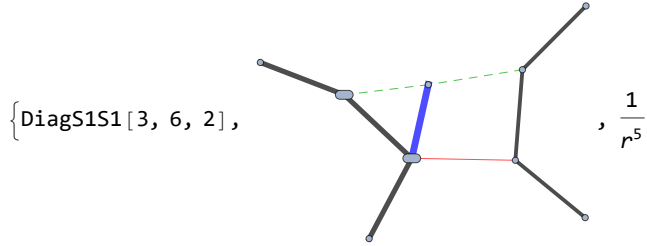
 $\left. , \frac{1}{r^5} \right\}$

$$\left\{ G^3 m_2^2 \left( -42 \hat{n} \times \vec{S}_1 \cdot \vec{v}_1 \hat{n} \times \vec{S}_1 \cdot \vec{v}_2 + 2 \vec{v}_1 \cdot \vec{v}_2 \left( \hat{n} \cdot \vec{S}_1 \right)^2 + 2 \hat{n} \cdot \vec{S}_1 \hat{n} \cdot \vec{v}_2 \vec{S}_1 \cdot \vec{v}_1 - 8 \hat{n} \cdot \vec{S}_1 \hat{n} \cdot \vec{v}_1 \vec{S}_1 \cdot \vec{v}_2 + 6 \vec{S}_1 \cdot \vec{S}_1 \hat{n} \cdot \vec{v}_1 \hat{n} \cdot \vec{v}_2 - 8 \vec{S}_1 \cdot \vec{v}_1 \vec{S}_1 \cdot \vec{v}_2 + 6 \vec{S}_1 \cdot \vec{S}_1 \vec{v}_1 \cdot \vec{v}_2 \right) \right\}$$

$\left\{ \text{DiagS1S1}[3, 6, 3], \right.$ 
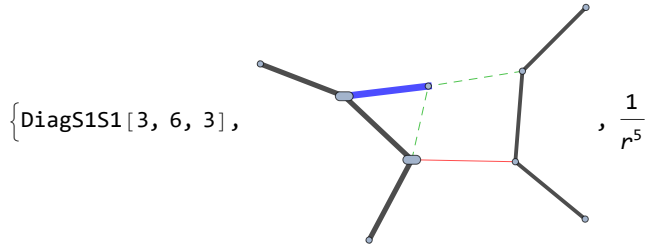
 $\left. , \frac{1}{r^5} \right\}$

$$\left\{ G^3 m_2^2 \left( 8 \vec{v}_1 \cdot \vec{v}_2 \left( \hat{n} \cdot \vec{S}_1 \right)^2 - 24 \hat{n} \cdot \vec{S}_1 \hat{n} \cdot \vec{v}_2 \vec{S}_1 \cdot \vec{v}_1 - 16 \hat{n} \cdot \vec{S}_1 \hat{n} \cdot \vec{v}_1 \vec{S}_1 \cdot \vec{v}_2 + 40 \vec{S}_1 \cdot \vec{S}_1 \hat{n} \cdot \vec{v}_1 \hat{n} \cdot \vec{v}_2 + 12 \vec{S}_1 \cdot \vec{v}_1 \vec{S}_1 \cdot \vec{v}_2 - 12 \vec{S}_1 \cdot \vec{S}_1 \vec{v}_1 \cdot \vec{v}_2 \right) \right\}$$

$\left\{ \text{DiagS1S1}[3, 6, 4], \right.$ 
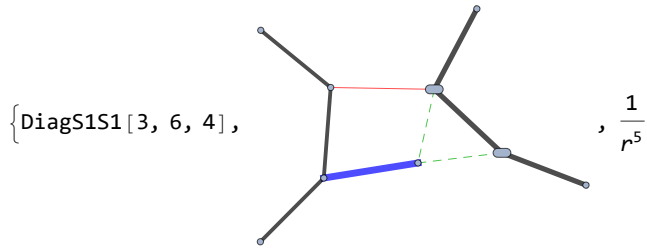
 $\left. , \frac{1}{r^5} \right\}$

$$\left\{ G^3 m_2^2 \left( 8 \left( \hat{n} \times \vec{S}_1 \cdot \vec{v}_2 \right)^2 - 18 \left( \hat{n} \cdot \vec{S}_1 \right)^2 \left( \hat{n} \cdot \vec{v}_2 \right)^2 + 14 \vec{S}_1 \cdot \vec{S}_1 \left( \hat{n} \cdot \vec{v}_2 \right)^2 - 8 \hat{n} \cdot \vec{S}_1 \hat{n} \cdot \vec{v}_2 \vec{S}_1 \cdot \vec{v}_2 + 14 \vec{v}_2 \cdot \vec{v}_2 \left( \hat{n} \cdot \vec{S}_1 \right)^2 + 8 \left( \vec{S}_1 \cdot \vec{v}_2 \right)^2 - 10 \vec{S}_1 \cdot \vec{S}_1 \vec{v}_2 \cdot \vec{v}_2 \right) \right\}$$

$\left\{ \text{DiagS1S1}[3, 6, 5], \right.$ 
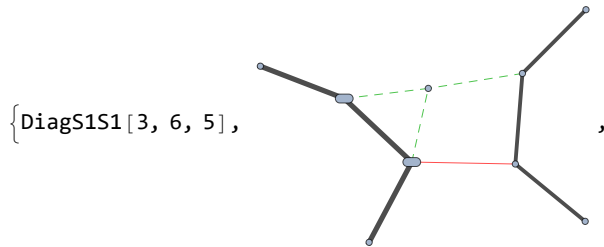
 $\left. , \right\}$

$$G^3 m_2^2 \left\{ \frac{8 \vec{S}_1 \cdot \vec{a}_2 \hat{n} \cdot \vec{S}_1 - 8 \vec{S}_1 \cdot \vec{S}_1 \hat{n} \cdot \vec{a}_2 - 16 \hat{n} \cdot \vec{S}_1 \hat{n} \cdot \vec{S}_1 \hat{n} \cdot \vec{v}_2}{r^4} + \frac{1}{r^5} \right. \\ \left. \left( 16 \hat{n} \times \vec{S}_1 \cdot \vec{v}_1 \hat{n} \times \vec{S}_1 \cdot \vec{v}_2 - 8 \left( \hat{n} \cdot \vec{S}_1 \right)^2 \left( \hat{n} \cdot \vec{v}_2 \right)^2 + 44 \left( \hat{n} \cdot \vec{S}_1 \right)^2 \hat{n} \cdot \vec{v}_1 \hat{n} \cdot \vec{v}_2 - \right. \right. \\ \left. 12 \vec{v}_1 \cdot \vec{v}_2 \left( \hat{n} \cdot \vec{S}_1 \right)^2 - 8 \hat{n} \cdot \vec{S}_1 \hat{n} \cdot \vec{v}_2 \vec{S}_1 \cdot \vec{v}_1 + 8 \hat{n} \cdot \vec{S}_1 \hat{n} \cdot \vec{v}_1 \vec{S}_1 \cdot \vec{v}_2 + 32 \hat{n} \cdot \vec{S}_1 \hat{n} \cdot \vec{v}_2 \vec{S}_1 \cdot \vec{v}_2 - \right. \\ \left. \left. 32 \vec{S}_1 \cdot \vec{S}_1 \left( \hat{n} \cdot \vec{v}_2 \right)^2 - 12 \vec{S}_1 \cdot \vec{S}_1 \hat{n} \cdot \vec{v}_1 \hat{n} \cdot \vec{v}_2 - 8 \left( \vec{S}_1 \cdot \vec{v}_2 \right)^2 + 4 \vec{S}_1 \cdot \vec{S}_1 \vec{v}_1 \cdot \vec{v}_2 + 8 \vec{S}_1 \cdot \vec{S}_1 \vec{v}_2 \cdot \vec{v}_2 \right) \right\}$$

{DiagS1S1[3, 6, 6],

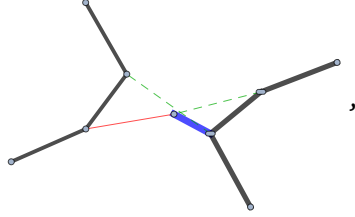

$$G^3 m_2^2 \left\{ \frac{1}{r^5} \left( -2 \hat{n} \times \vec{S}_1 \cdot \vec{v}_1 \hat{n} \times \vec{S}_1 \cdot \vec{v}_2 + 24 \left( \hat{n} \cdot \vec{S}_1 \right)^2 \left( \hat{n} \cdot \vec{v}_2 \right)^2 - 24 \left( \hat{n} \cdot \vec{S}_1 \right)^2 \hat{n} \cdot \vec{v}_1 \hat{n} \cdot \vec{v}_2 + 6 \vec{v}_1 \cdot \vec{v}_2 \left( \hat{n} \cdot \vec{S}_1 \right)^2 - \right. \right. \\ \left. 6 \vec{v}_2 \cdot \vec{v}_2 \left( \hat{n} \cdot \vec{S}_1 \right)^2 + 4 \hat{n} \cdot \vec{S}_1 \hat{n} \cdot \vec{v}_2 \vec{S}_1 \cdot \vec{v}_1 + 18 \hat{n} \cdot \vec{S}_1 \hat{n} \cdot \vec{v}_1 \vec{S}_1 \cdot \vec{v}_2 - 24 \hat{n} \cdot \vec{S}_1 \hat{n} \cdot \vec{v}_2 \vec{S}_1 \cdot \vec{v}_2 + \right. \\ \left. \left. 2 \vec{S}_1 \cdot \vec{S}_1 \hat{n} \cdot \vec{v}_1 \hat{n} \cdot \vec{v}_2 + 6 \left( \vec{S}_1 \cdot \vec{v}_2 \right)^2 - 4 \vec{S}_1 \cdot \vec{v}_1 \vec{S}_1 \cdot \vec{v}_2 - 2 \vec{S}_1 \cdot \vec{S}_1 \vec{v}_1 \cdot \vec{v}_2 \right) + \frac{8 \hat{n} \cdot \vec{S}_1 \hat{n} \cdot \vec{S}_1 \hat{n} \cdot \vec{v}_2 - 8 \hat{n} \cdot \vec{S}_1 \vec{S}_1 \cdot \vec{v}_2}{r^4} \right\}$$

{DiagS1S1[3, 6, 7],

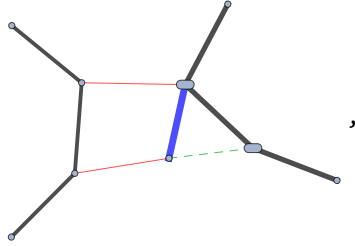

$$G^3 m_2^2 \left\{ \frac{1}{r^5} \left( -10 \left( \hat{n} \times \vec{S}_1 \cdot \vec{v}_1 \right)^2 + 12 \hat{n} \times \vec{S}_1 \cdot \vec{v}_2 \hat{n} \times \vec{S}_1 \cdot \vec{v}_1 - 24 \left( \hat{n} \cdot \vec{S}_1 \right)^2 \left( \hat{n} \cdot \vec{v}_1 \right)^2 + 24 \left( \hat{n} \cdot \vec{S}_1 \right)^2 \hat{n} \cdot \vec{v}_1 \hat{n} \cdot \vec{v}_2 + \right. \right. \\ \left. 38 \vec{S}_1 \cdot \vec{S}_1 \left( \hat{n} \cdot \vec{v}_1 \right)^2 - 36 \vec{S}_1 \cdot \vec{S}_1 \hat{n} \cdot \vec{v}_1 \hat{n} \cdot \vec{v}_2 - 14 \hat{n} \cdot \vec{S}_1 \hat{n} \cdot \vec{v}_1 \vec{S}_1 \cdot \vec{v}_1 + 18 \hat{n} \cdot \vec{S}_1 \hat{n} \cdot \vec{v}_2 \vec{S}_1 \cdot \vec{v}_1 - 6 \hat{n} \cdot \vec{S}_1 \hat{n} \cdot \vec{v}_1 \vec{S}_1 \cdot \vec{v}_2 + \right. \\ \left. 6 \vec{v}_1 \cdot \vec{v}_1 \left( \hat{n} \cdot \vec{S}_1 \right)^2 - 6 \vec{v}_1 \cdot \vec{v}_2 \left( \hat{n} \cdot \vec{S}_1 \right)^2 + 4 \left( \vec{S}_1 \cdot \vec{v}_1 \right)^2 - 6 \vec{S}_1 \cdot \vec{v}_1 \vec{S}_1 \cdot \vec{v}_2 - 10 \vec{S}_1 \cdot \vec{S}_1 \vec{v}_1 \cdot \vec{v}_1 + 12 \vec{S}_1 \cdot \vec{S}_1 \vec{v}_1 \cdot \vec{v}_2 \right) + \right. \\ \left. \frac{8 \hat{n} \cdot \vec{S}_1 \hat{n} \cdot \vec{S}_1 \hat{n} \cdot \vec{v}_1 - 16 \vec{S}_1 \cdot \vec{S}_1 \hat{n} \cdot \vec{v}_1 + 8 \hat{n} \cdot \vec{S}_1 \vec{S}_1 \cdot \vec{v}_1}{r^4} \right\}$$

{DiagS1S1[3, 6, 8],

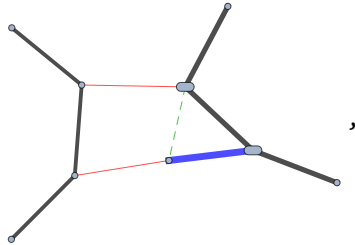

$$G^3 m_2^2 \left\{ \frac{1}{r^5} \left( -8 \left( \hat{n} \times \vec{S}_1 \cdot \vec{v}_1 \right)^2 + 64 \left( \hat{n} \cdot \vec{S}_1 \right)^2 \left( \hat{n} \cdot \vec{v}_1 \right)^2 - 64 \left( \hat{n} \cdot \vec{S}_1 \right)^2 \hat{n} \cdot \vec{v}_1 \hat{n} \cdot \vec{v}_2 + 36 \vec{S}_1 \cdot \vec{S}_1 \left( \hat{n} \cdot \vec{v}_1 \right)^2 - \right. \right. \\ \left. \left. 44 \vec{S}_1 \cdot \vec{S}_1 \hat{n} \cdot \vec{v}_1 \hat{n} \cdot \vec{v}_2 - 52 \hat{n} \cdot \vec{S}_1 \hat{n} \cdot \vec{v}_1 \vec{S}_1 \cdot \vec{v}_1 + 44 \hat{n} \cdot \vec{S}_1 \hat{n} \cdot \vec{v}_2 \vec{S}_1 \cdot \vec{v}_1 + 16 \hat{n} \cdot \vec{S}_1 \hat{n} \cdot \vec{v}_1 \vec{S}_1 \cdot \vec{v}_2 - \right. \right. \\ \left. \left. 8 \vec{v}_1 \cdot \vec{v}_1 \left( \hat{n} \cdot \vec{S}_1 \right)^2 + 8 \vec{v}_1 \cdot \vec{v}_2 \left( \hat{n} \cdot \vec{S}_1 \right)^2 + 4 \left( \vec{S}_1 \cdot \vec{v}_1 \right)^2 - 8 \vec{S}_1 \cdot \vec{v}_1 \vec{S}_1 \cdot \vec{v}_2 - 4 \vec{S}_1 \cdot \vec{S}_1 \vec{v}_1 \cdot \vec{v}_1 + 8 \vec{S}_1 \cdot \vec{S}_1 \vec{v}_1 \cdot \vec{v}_2 \right) + \right. \\ \left. \frac{-16 \hat{n} \cdot \vec{S}_1 \hat{n} \cdot \vec{S}_1 \hat{n} \cdot \vec{v}_1 - 12 \vec{S}_1 \cdot \vec{S}_1 \hat{n} \cdot \vec{v}_1 + 4 \hat{n} \cdot \vec{S}_1 \vec{S}_1 \cdot \vec{v}_1 + 8 \hat{n} \cdot \vec{S}_1 \vec{S}_1 \cdot \vec{v}_1}{r^4} \right\}$$

{DiagS1S1[3, 6, 9],

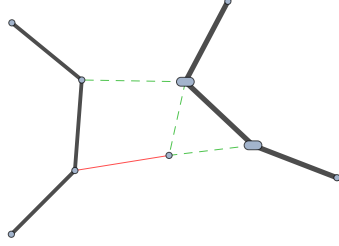

,

$$G^3 m_2^2 \left\{ \frac{4 \vec{S}_1 \cdot \vec{a}_2 \hat{n} \cdot \vec{S}_1 - 4 \vec{S}_1 \cdot \vec{S}_1 \hat{n} \cdot \vec{a}_2 - 4 \hat{n} \cdot \vec{S}_1 \vec{S}_1 \cdot \vec{v}_2 + 4 \vec{S}_1 \cdot \vec{S}_1 \hat{n} \cdot \vec{v}_2}{r^4} + \frac{1}{r^5} \right. \\ \left. \left( -4 \hat{n} \times \vec{S}_1 \cdot \vec{v}_1 \hat{n} \times \vec{S}_1 \cdot \vec{v}_2 + 8 \vec{v}_1 \cdot \vec{v}_2 \left( \hat{n} \cdot \vec{S}_1 \right)^2 + 16 \hat{n} \cdot \vec{S}_1 \hat{n} \cdot \vec{v}_1 \vec{S}_1 \cdot \vec{v}_2 - 12 \hat{n} \cdot \vec{S}_1 \hat{n} \cdot \vec{v}_2 \vec{S}_1 \cdot \vec{v}_2 + 12 \vec{S}_1 \cdot \vec{S}_1 \left( \hat{n} \cdot \vec{v}_2 \right)^2 - \right. \right. \\ \left. \left. 16 \vec{S}_1 \cdot \vec{S}_1 \hat{n} \cdot \vec{v}_1 \hat{n} \cdot \vec{v}_2 + 4 \left( \vec{S}_1 \cdot \vec{v}_2 \right)^2 - 8 \vec{S}_1 \cdot \vec{v}_1 \vec{S}_1 \cdot \vec{v}_2 + 8 \vec{S}_1 \cdot \vec{S}_1 \vec{v}_1 \cdot \vec{v}_2 - 4 \vec{S}_1 \cdot \vec{S}_1 \vec{v}_2 \cdot \vec{v}_2 \right) \right\}$$

{DiagS1S1[3, 6, 10],

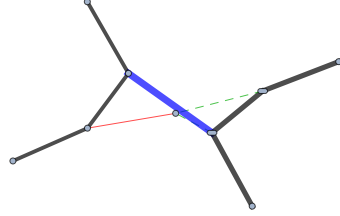

,

$$\frac{G^3 m_2^2 \left( 4 \left( \hat{n} \times \vec{S}_1 \cdot \vec{v}_2 \right)^2 + 4 \vec{S}_1 \cdot \vec{S}_1 \left( \hat{n} \cdot \vec{v}_2 \right)^2 - 4 \hat{n} \cdot \vec{S}_1 \hat{n} \cdot \vec{v}_2 \vec{S}_1 \cdot \vec{v}_2 + 8 \vec{v}_2 \cdot \vec{v}_2 \left( \hat{n} \cdot \vec{S}_1 \right)^2 + 4 \left( \vec{S}_1 \cdot \vec{v}_2 \right)^2 - 4 \vec{S}_1 \cdot \vec{S}_1 \vec{v}_2 \cdot \vec{v}_2 \right)}{r^5}$$

{DiagS1S1[3, 6, 11],

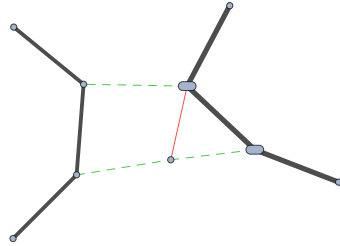

$$, - \frac{16 G^3 m_2^2 \left( \hat{n} \times \vec{S}_1 \cdot \vec{v}_2 \right)^2}{r^5}$$

{DiagS1S1[3, 6, 12],

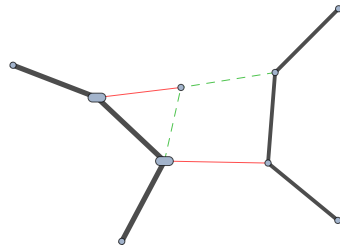

,

$$\frac{G^3 m_2^2 \left( -32 \vec{S}_1 \cdot \vec{S}_1 \hat{n} \cdot \vec{v}_1 \hat{n} \cdot \vec{v}_2 + 32 \hat{n} \cdot \vec{S}_1 \hat{n} \cdot \vec{v}_2 \vec{S}_1 \cdot \vec{v}_1 + 16 \vec{S}_1 \cdot \vec{S}_1 \vec{v}_1 \cdot \vec{v}_2 - 16 \vec{S}_1 \cdot \vec{v}_1 \vec{S}_1 \cdot \vec{v}_2 \right)}{r^5} \Bigg\}$$

$$\left\{ \text{DiagS1S1}[3, 6, 13], \frac{16 G^3 m_2^2 \hat{n} \times \vec{S}_1 \cdot \vec{v}_1 \hat{n} \times \vec{S}_1 \cdot \vec{v}_2}{r^5} \right\}$$
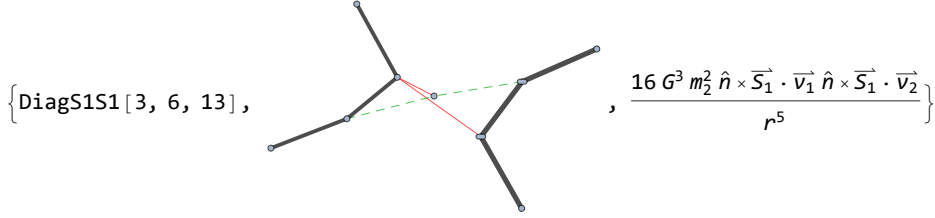

$$\left\{ \text{DiagS1S1}[3, 6, 14], -\frac{16 G^3 m_2^2 \left( \hat{n} \times \vec{S}_1 \cdot \vec{v}_2 \right)^2}{r^5} \right\}$$
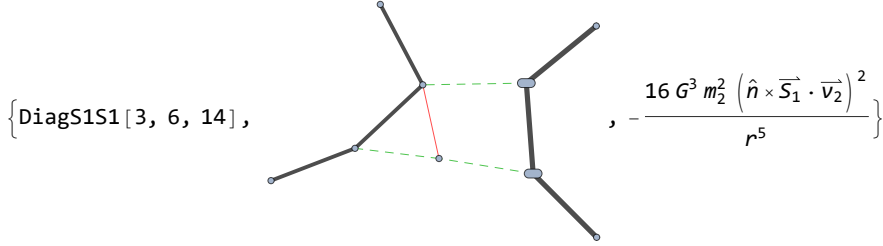

$$\left\{ \text{DiagS1S1}[3, 6, 15], \frac{16 G^3 m_2^2 \hat{n} \times \vec{S}_1 \cdot \vec{v}_1 \hat{n} \times \vec{S}_1 \cdot \vec{v}_2}{r^5} \right\}$$
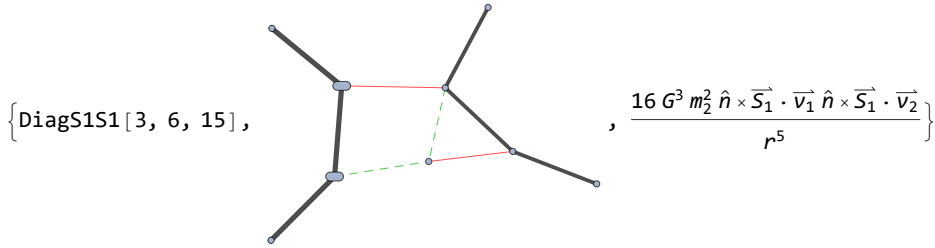

$$\left\{ \text{DiagS1S1}[3, 6, 16], \right\}$$
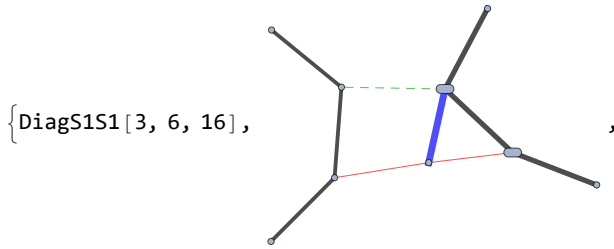

$$\frac{G^3 m_2^2 \left( -14 \hat{n} \times \vec{S}_1 \cdot \vec{v}_1 \hat{n} \times \vec{S}_1 \cdot \vec{v}_2 - 10 \vec{S}_1 \cdot \vec{S}_1 \hat{n} \cdot \vec{v}_1 \hat{n} \cdot \vec{v}_2 + 10 \hat{n} \cdot \vec{S}_1 \hat{n} \cdot \vec{v}_2 \vec{S}_1 \cdot \vec{v}_1 - 10 \vec{S}_1 \cdot \vec{v}_1 \vec{S}_1 \cdot \vec{v}_2 + 10 \vec{S}_1 \cdot \vec{S}_1 \vec{v}_1 \cdot \vec{v}_2 \right)}{r^5} \Bigg\}$$

$$\left\{ \text{DiagS1S1}[3, 6, 17], \right\}$$
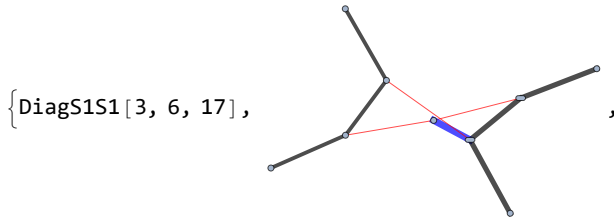

$$\frac{G^3 m_2^2 \left( 38 \left( \hat{n} \times \vec{S}_1 \cdot \vec{v}_1 \right)^2 - 10 \vec{S}_1 \cdot \vec{S}_1 \left( \hat{n} \cdot \vec{v}_1 \right)^2 + 10 \hat{n} \cdot \vec{S}_1 \hat{n} \cdot \vec{v}_1 \vec{S}_1 \cdot \vec{v}_1 + 10 \left( \vec{S}_1 \cdot \vec{v}_1 \right)^2 - 10 \vec{S}_1 \cdot \vec{S}_1 \vec{v}_1 \cdot \vec{v}_1 \right)}{r^5} \Bigg\}$$

{DiagS1S1[3, 6, 18],

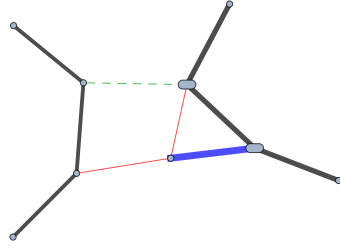

$$, - \frac{4 G^3 m_2^2 \hat{n} \times \vec{S}_1 \cdot \vec{v}_1 \hat{n} \times \vec{S}_1 \cdot \vec{v}_2}{r^5} \}$$

{DiagS1S1[3, 6, 19],

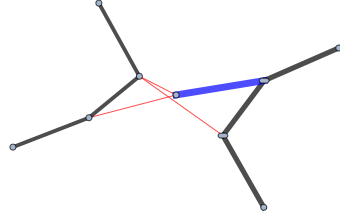

$$, \frac{2 G^3 m_2^2 \left( \hat{n} \times \vec{S}_1 \cdot \vec{v}_1 \right)^2}{r^5} \}$$

{DiagS1S1[3, 6, 20],

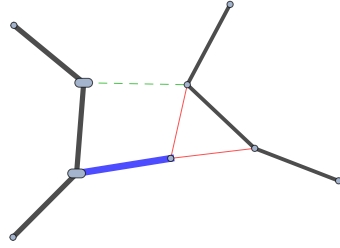

$$, - \frac{2 G^3 m_2^2 \hat{n} \times \vec{S}_1 \cdot \vec{v}_1 \hat{n} \times \vec{S}_1 \cdot \vec{v}_2}{r^5} \}$$

{DiagS1S1[3, 6, 21],

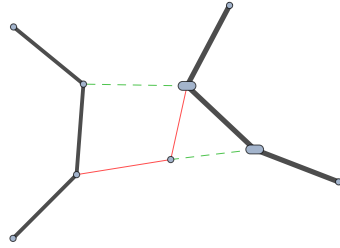

$$, \frac{4 G^3 m_2^2 \hat{n} \times \vec{S}_1 \cdot \vec{v}_1 \hat{n} \times \vec{S}_1 \cdot \vec{v}_2}{r^5} \}$$

{DiagS1S1[3, 6, 22],

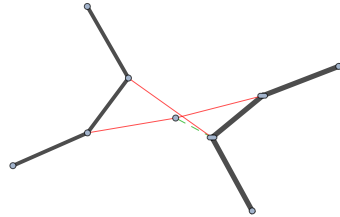

,

$$G^3 m_2^2 \left( \frac{4 \vec{S}_1 \cdot \vec{a}_1 \hat{n} \cdot \vec{S}_1 - 4 \vec{S}_1 \cdot \vec{S}_1 \hat{n} \cdot \vec{a}_1 - 4 \vec{S}_1 \cdot \vec{S}_1 \hat{n} \cdot \vec{v}_1 + 4 \hat{n} \cdot \vec{S}_1 \vec{S}_1 \cdot \vec{v}_1}{r^4} + \frac{1}{r^5} \left( -8 \left( \hat{n} \times \vec{S}_1 \cdot \vec{v}_1 \right)^2 + 8 \vec{S}_1 \cdot \vec{S}_1 \left( \hat{n} \cdot \vec{v}_1 \right)^2 + \right. \right. \\ \left. \left. 16 \vec{S}_1 \cdot \vec{S}_1 \hat{n} \cdot \vec{v}_1 \hat{n} \cdot \vec{v}_2 - 8 \hat{n} \cdot \vec{S}_1 \hat{n} \cdot \vec{v}_1 \vec{S}_1 \cdot \vec{v}_1 - 16 \hat{n} \cdot \vec{S}_1 \hat{n} \cdot \vec{v}_2 \vec{S}_1 \cdot \vec{v}_1 + 4 \vec{S}_1 \cdot \vec{v}_1 \vec{S}_1 \cdot \vec{v}_2 - 4 \vec{S}_1 \cdot \vec{S}_1 \vec{v}_1 \cdot \vec{v}_2 \right) \right) \}$$

{DiagS1S1[3, 6, 23],

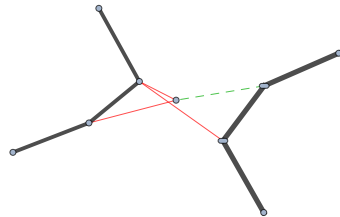

$$, - \frac{2 G^3 m_2^2 \hat{n} \times \vec{S}_1 \cdot \vec{v}_1 \hat{n} \times \vec{S}_1 \cdot \vec{v}_2}{r^5} \}$$

{DiagS1S1[3, 6, 24],

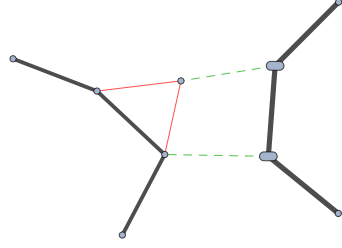

$$, \frac{2 G^3 m_2^2 \left( \hat{n} \times \vec{S}_1 \cdot \vec{v}_2 \right)^2}{r^5} \}$$

{DiagS1S1[3, 6, 25],

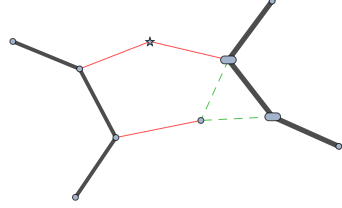

$$, G^3 m_2^2$$

$$\left( \frac{-24 \left( \hat{n} \cdot \vec{S}_1 \right)^2 \left( \hat{n} \cdot \vec{v}_2 \right)^2 + 28 \left( \hat{n} \cdot \vec{S}_1 \right)^2 \hat{n} \cdot \vec{v}_1 \hat{n} \cdot \vec{v}_2 - 4 \vec{v}_1 \cdot \vec{v}_2 \left( \hat{n} \cdot \vec{S}_1 \right)^2 - 8 \hat{n} \cdot \vec{S}_1 \hat{n} \cdot \vec{v}_2 \vec{S}_1 \cdot \vec{v}_1 + 8 \hat{n} \cdot \vec{S}_1 \hat{n} \cdot \vec{v}_2 \vec{S}_1 \cdot \vec{v}_2}{r^5} - \frac{8 \hat{n} \cdot \vec{S}_1 \hat{n} \cdot \vec{S}_1 \hat{n} \cdot \vec{v}_2}{r^4} \right) \}$$

{DiagS1S1[3, 6, 26],

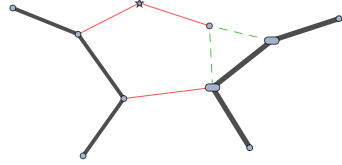

,

$$G^3 m_2^2 \left( \frac{1}{r^5} \left( -8 \left( \hat{n} \cdot \vec{S}_1 \right)^2 \left( \hat{n} \cdot \vec{v}_2 \right)^2 + 56 \left( \hat{n} \cdot \vec{S}_1 \right)^2 \hat{n} \cdot \vec{v}_1 \hat{n} \cdot \vec{v}_2 - 8 \vec{v}_1 \cdot \vec{v}_2 \left( \hat{n} \cdot \vec{S}_1 \right)^2 - 16 \hat{n} \cdot \vec{S}_1 \hat{n} \cdot \vec{v}_2 \vec{S}_1 \cdot \vec{v}_1 - 20 \hat{n} \cdot \vec{S}_1 \hat{n} \cdot \vec{v}_1 \vec{S}_1 \cdot \vec{v}_2 + 4 \hat{n} \cdot \vec{S}_1 \hat{n} \cdot \vec{v}_2 \vec{S}_1 \cdot \vec{v}_2 + 4 \vec{S}_1 \cdot \vec{S}_1 \left( \hat{n} \cdot \vec{v}_2 \right)^2 - 20 \vec{S}_1 \cdot \vec{S}_1 \hat{n} \cdot \vec{v}_1 \hat{n} \cdot \vec{v}_2 + 4 \vec{S}_1 \cdot \vec{v}_1 \vec{S}_1 \cdot \vec{v}_2 + 4 \vec{S}_1 \cdot \vec{S}_1 \vec{v}_1 \cdot \vec{v}_2 \right) + \frac{-16 \hat{n} \cdot \vec{S}_1 \hat{n} \cdot \vec{S}_1 \hat{n} \cdot \vec{v}_2 + 8 \vec{S}_1 \cdot \vec{S}_1 \hat{n} \cdot \vec{v}_2 + 4 \hat{n} \cdot \vec{S}_1 \vec{S}_1 \cdot \vec{v}_2 + 4 \hat{n} \cdot \vec{S}_1 \vec{S}_1 \cdot \vec{v}_2}{r^4} \right) \}$$

{DiagS1S1[3, 6, 27],

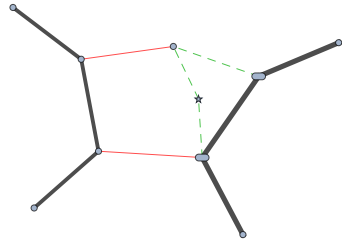

,

$$G^3 m_2^2 \left( \frac{1}{r^5} \left( 8 \left( \hat{n} \times \vec{S}_1 \cdot \vec{v}_1 \right)^2 + 59 \left( \hat{n} \cdot \vec{S}_1 \right)^2 \left( \hat{n} \cdot \vec{v}_1 \right)^2 + 40 \left( \hat{n} \cdot \vec{S}_1 \right)^2 \left( \hat{n} \cdot \vec{v}_2 \right)^2 - 120 \left( \hat{n} \cdot \vec{S}_1 \right)^2 \hat{n} \cdot \vec{v}_1 \hat{n} \cdot \vec{v}_2 - 7 \vec{S}_1 \cdot \vec{S}_1 \left( \hat{n} \cdot \vec{v}_1 \right)^2 - 12 \vec{S}_1 \cdot \vec{S}_1 \left( \hat{n} \cdot \vec{v}_2 \right)^2 + 30 \vec{S}_1 \cdot \vec{S}_1 \hat{n} \cdot \vec{v}_1 \hat{n} \cdot \vec{v}_2 - 42 \hat{n} \cdot \vec{S}_1 \hat{n} \cdot \vec{v}_1 \vec{S}_1 \cdot \vec{v}_1 + 38 \hat{n} \cdot \vec{S}_1 \hat{n} \cdot \vec{v}_2 \vec{S}_1 \cdot \vec{v}_1 + 36 \hat{n} \cdot \vec{S}_1 \hat{n} \cdot \vec{v}_1 \vec{S}_1 \cdot \vec{v}_2 - 20 \hat{n} \cdot \vec{S}_1 \hat{n} \cdot \vec{v}_2 \vec{S}_1 \cdot \vec{v}_2 - 5 \vec{v}_1 \cdot \vec{v}_1 \left( \hat{n} \cdot \vec{S}_1 \right)^2 + 8 \vec{v}_1 \cdot \vec{v}_2 \left( \hat{n} \cdot \vec{S}_1 \right)^2 + 8 \left( \vec{S}_1 \cdot \vec{v}_1 \right)^2 - 6 \vec{S}_1 \cdot \vec{v}_1 \vec{S}_1 \cdot \vec{v}_2 - 5 \vec{S}_1 \cdot \vec{S}_1 \vec{v}_1 \cdot \vec{v}_1 - 2 \vec{S}_1 \cdot \vec{S}_1 \vec{v}_1 \cdot \vec{v}_2 \right) + \frac{1}{r^4} \right)$$

$$\left( -50 \hat{n} \cdot \vec{S}_1 \hat{n} \cdot \vec{S}_1 \hat{n} \cdot \vec{v}_1 + 18 \vec{S}_1 \cdot \vec{S}_1 \hat{n} \cdot \vec{v}_1 + 50 \hat{n} \cdot \vec{S}_1 \hat{n} \cdot \vec{S}_1 \hat{n} \cdot \vec{v}_2 + 16 \hat{n} \cdot \vec{S}_1 \vec{S}_1 \cdot \vec{v}_1 - 10 \hat{n} \cdot \vec{S}_1 \vec{S}_1 \cdot \vec{v}_2 - \right. \\ \left. 18 \vec{S}_1 \cdot \vec{S}_1 \hat{n} \cdot \vec{v}_2 + 4 \hat{n} \cdot \vec{S}_1 \vec{S}_1 \cdot \vec{v}_1 - 10 \hat{n} \cdot \vec{S}_1 \vec{S}_1 \cdot \vec{v}_2 \right) + \frac{10 \left( \hat{n} \cdot \vec{S}_1 \right)^2 - 6 \vec{S}_1 \cdot \vec{S}_1}{r^3} \Bigg\}$$

{DiagS1S1[3, 6, 28],

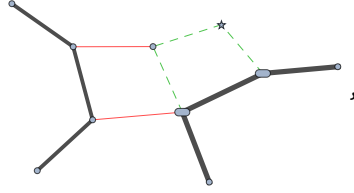

$$G^3 m_2^2 \left\{ \frac{1}{r^5} \left( 8 \left( \hat{n} \times \vec{S}_1 \cdot \vec{v}_1 \right)^2 + 35 \left( \hat{n} \cdot \vec{S}_1 \right)^2 \left( \hat{n} \cdot \vec{v}_1 \right)^2 - 56 \left( \hat{n} \cdot \vec{S}_1 \right)^2 \hat{n} \cdot \vec{v}_1 \hat{n} \cdot \vec{v}_2 + \vec{S}_1 \cdot \vec{S}_1 \left( \hat{n} \cdot \vec{v}_1 \right)^2 + \right. \right. \\ \left. 10 \vec{S}_1 \cdot \vec{S}_1 \hat{n} \cdot \vec{v}_1 \hat{n} \cdot \vec{v}_2 - 34 \hat{n} \cdot \vec{S}_1 \hat{n} \cdot \vec{v}_1 \vec{S}_1 \cdot \vec{v}_1 + 30 \hat{n} \cdot \vec{S}_1 \hat{n} \cdot \vec{v}_2 \vec{S}_1 \cdot \vec{v}_1 + 16 \hat{n} \cdot \vec{S}_1 \hat{n} \cdot \vec{v}_1 \vec{S}_1 \cdot \vec{v}_2 - \right. \\ \left. 5 \vec{v}_1 \cdot \vec{v}_1 \left( \hat{n} \cdot \vec{S}_1 \right)^2 + 8 \vec{v}_1 \cdot \vec{v}_2 \left( \hat{n} \cdot \vec{S}_1 \right)^2 + 8 \left( \vec{S}_1 \cdot \vec{v}_1 \right)^2 - 6 \vec{S}_1 \cdot \vec{v}_1 \vec{S}_1 \cdot \vec{v}_2 - 5 \vec{S}_1 \cdot \vec{S}_1 \vec{v}_1 \cdot \vec{v}_1 - 2 \vec{S}_1 \cdot \vec{S}_1 \vec{v}_1 \cdot \vec{v}_2 \right) + \\ \left. \frac{1}{r^4} \left( -50 \hat{n} \cdot \vec{S}_1 \hat{n} \cdot \vec{S}_1 \hat{n} \cdot \vec{v}_1 + 18 \vec{S}_1 \cdot \vec{S}_1 \hat{n} \cdot \vec{v}_1 + 50 \hat{n} \cdot \vec{S}_1 \hat{n} \cdot \vec{S}_1 \hat{n} \cdot \vec{v}_2 + 16 \hat{n} \cdot \vec{S}_1 \vec{S}_1 \cdot \vec{v}_1 - 10 \hat{n} \cdot \vec{S}_1 \vec{S}_1 \cdot \vec{v}_2 - \right. \right. \\ \left. 18 \vec{S}_1 \cdot \vec{S}_1 \hat{n} \cdot \vec{v}_2 + 4 \hat{n} \cdot \vec{S}_1 \vec{S}_1 \cdot \vec{v}_1 - 10 \hat{n} \cdot \vec{S}_1 \vec{S}_1 \cdot \vec{v}_2 \right) + \frac{10 \left( \hat{n} \cdot \vec{S}_1 \right)^2 - 6 \vec{S}_1 \cdot \vec{S}_1}{r^3} \Bigg\}$$

{DiagS1S1[3, 6, 29],

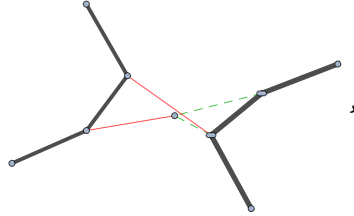

$$G^3 m_2^2 \left\{ \frac{8 \vec{S}_1 \cdot \vec{a}_1 \hat{n} \cdot \vec{S}_1 - 8 \vec{S}_1 \cdot \vec{S}_1 \hat{n} \cdot \vec{a}_1 - 8 \vec{S}_1 \cdot \vec{S}_1 \hat{n} \cdot \vec{v}_1 + 8 \hat{n} \cdot \vec{S}_1 \vec{S}_1 \cdot \vec{v}_1}{r^4} + \frac{1}{r^5} \right. \\ \left( -4 \left( \hat{n} \times \vec{S}_1 \cdot \vec{v}_1 \right)^2 + 12 \vec{S}_1 \cdot \vec{S}_1 \left( \hat{n} \cdot \vec{v}_1 \right)^2 + 4 \vec{S}_1 \cdot \vec{S}_1 \hat{n} \cdot \vec{v}_1 \hat{n} \cdot \vec{v}_2 - 12 \hat{n} \cdot \vec{S}_1 \hat{n} \cdot \vec{v}_1 \vec{S}_1 \cdot \vec{v}_1 - \right. \\ \left. 4 \hat{n} \cdot \vec{S}_1 \hat{n} \cdot \vec{v}_2 \vec{S}_1 \cdot \vec{v}_1 - 24 \vec{v}_2 \cdot \vec{v}_2 \left( \hat{n} \cdot \vec{S}_1 \right)^2 + 4 \left( \vec{S}_1 \cdot \vec{v}_1 \right)^2 - 4 \vec{S}_1 \cdot \vec{S}_1 \vec{v}_1 \cdot \vec{v}_1 \right) \Bigg\}$$

{DiagS1S1[3, 7, 1],

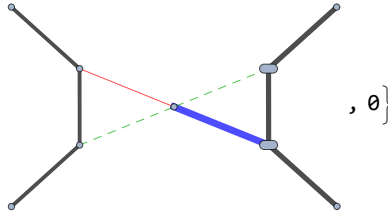

, 0}

$\{\text{DiagS1S1}[3, 7, 2],$ 
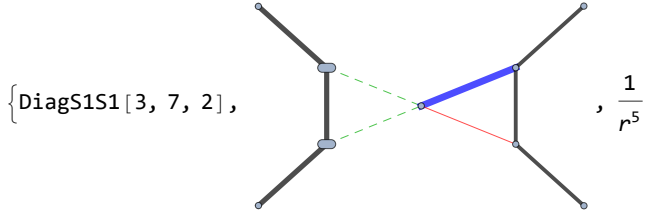
 $, \frac{1}{r^5}$

$$\pi^2 G^3 m_2^2 \left( -\frac{315}{64} (\hat{n} \cdot \vec{S}_1)^2 (\hat{n} \cdot \vec{v}_2)^2 + \frac{45}{64} \vec{v}_2 \cdot \vec{v}_2 (\hat{n} \cdot \vec{S}_1)^2 + \frac{45}{16} \hat{n} \cdot \vec{S}_1 \hat{n} \cdot \vec{v}_2 \vec{S}_1 \cdot \vec{v}_2 + \right. \\ \left. \frac{45}{64} \vec{S}_1 \cdot \vec{S}_1 (\hat{n} \cdot \vec{v}_2)^2 - \frac{9}{32} (\vec{S}_1 \cdot \vec{v}_2)^2 - \frac{9}{64} \vec{S}_1 \cdot \vec{S}_1 \vec{v}_2 \cdot \vec{v}_2 \right) \}$$

$\{\text{DiagS1S1}[3, 7, 3],$ 
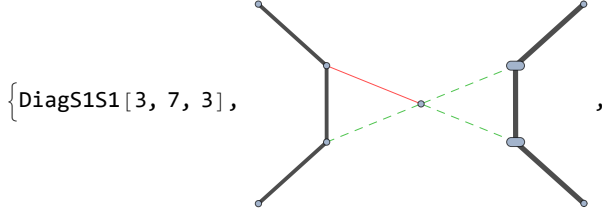
 $,$

$$\pi^2 G^3 m_2^2 \left( \frac{\frac{15}{4} \hat{n} \cdot \vec{a}_2 (\hat{n} \cdot \vec{S}_1)^2 - \frac{3}{2} \vec{S}_1 \cdot \vec{a}_2 \hat{n} \cdot \vec{S}_1 - \frac{3}{4} \vec{S}_1 \cdot \vec{S}_1 \hat{n} \cdot \vec{a}_2}{r^4} + \frac{1}{r^5} \right. \\ \left( \frac{105}{8} (\hat{n} \cdot \vec{S}_1)^2 (\hat{n} \cdot \vec{v}_2)^2 - \frac{105}{32} (\hat{n} \cdot \vec{S}_1)^2 \hat{n} \cdot \vec{v}_1 \hat{n} \cdot \vec{v}_2 + \frac{15}{32} \vec{v}_1 \cdot \vec{v}_2 (\hat{n} \cdot \vec{S}_1)^2 - \frac{15}{8} \vec{v}_2 \cdot \vec{v}_2 (\hat{n} \cdot \vec{S}_1)^2 + \right. \\ \left. \frac{15}{16} \hat{n} \cdot \vec{S}_1 \hat{n} \cdot \vec{v}_2 \vec{S}_1 \cdot \vec{v}_1 + \frac{15}{16} \hat{n} \cdot \vec{S}_1 \hat{n} \cdot \vec{v}_1 \vec{S}_1 \cdot \vec{v}_2 - \frac{15}{2} \hat{n} \cdot \vec{S}_1 \hat{n} \cdot \vec{v}_2 \vec{S}_1 \cdot \vec{v}_2 - \frac{15}{8} \vec{S}_1 \cdot \vec{S}_1 (\hat{n} \cdot \vec{v}_2)^2 + \right. \\ \left. \left. \frac{15}{32} \vec{S}_1 \cdot \vec{S}_1 \hat{n} \cdot \vec{v}_1 \hat{n} \cdot \vec{v}_2 + \frac{3}{4} (\vec{S}_1 \cdot \vec{v}_2)^2 - \frac{3}{16} \vec{S}_1 \cdot \vec{v}_1 \vec{S}_1 \cdot \vec{v}_2 - \frac{3}{32} \vec{S}_1 \cdot \vec{S}_1 \vec{v}_1 \cdot \vec{v}_2 + \frac{3}{8} \vec{S}_1 \cdot \vec{S}_1 \vec{v}_2 \cdot \vec{v}_2 \right) \right) \}$$

$\{\text{DiagS1S1}[3, 7, 4],$ 
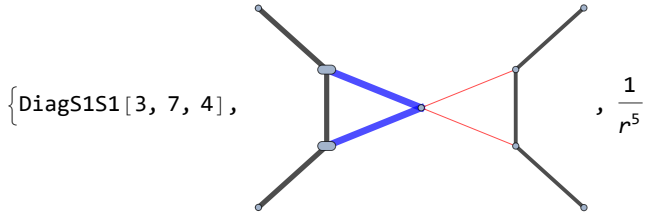
 $, \frac{1}{r^5}$

$$\pi^2 G^3 m_2^2 \left( \frac{105}{128} (\hat{n} \cdot \vec{S}_1)^2 (\hat{n} \cdot \vec{v}_1)^2 - \frac{15}{128} \vec{v}_1 \cdot \vec{v}_1 (\hat{n} \cdot \vec{S}_1)^2 - \frac{15}{32} \hat{n} \cdot \vec{S}_1 \hat{n} \cdot \vec{v}_1 \vec{S}_1 \cdot \vec{v}_1 - \right. \\ \left. \frac{15}{128} \vec{S}_1 \cdot \vec{S}_1 (\hat{n} \cdot \vec{v}_1)^2 + \frac{3}{64} (\vec{S}_1 \cdot \vec{v}_1)^2 + \frac{3}{128} \vec{S}_1 \cdot \vec{S}_1 \vec{v}_1 \cdot \vec{v}_1 \right) \}$$

$\{\text{DiagS1S1}[3, 7, 5],$ 
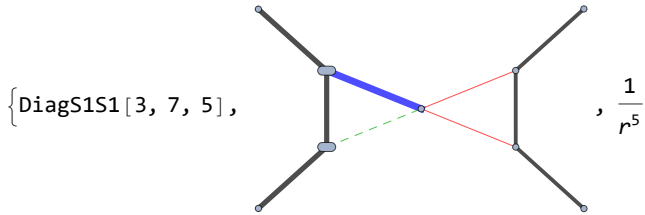
 $, \frac{1}{r^5}$

$$\pi^2 G^3 m_2^2 \left( -\frac{105}{64} (\hat{n} \cdot \vec{S}_1)^2 \hat{n} \cdot \vec{v}_1 \hat{n} \cdot \vec{v}_2 + \frac{15}{64} \vec{v}_1 \cdot \vec{v}_2 (\hat{n} \cdot \vec{S}_1)^2 + \frac{15}{32} \hat{n} \cdot \vec{S}_1 \hat{n} \cdot \vec{v}_2 \vec{S}_1 \cdot \vec{v}_1 + \right. \\ \left. \frac{15}{32} \hat{n} \cdot \vec{S}_1 \hat{n} \cdot \vec{v}_1 \vec{S}_1 \cdot \vec{v}_2 + \frac{15}{64} \vec{S}_1 \cdot \vec{S}_1 \hat{n} \cdot \vec{v}_1 \hat{n} \cdot \vec{v}_2 - \frac{3}{32} \vec{S}_1 \cdot \vec{v}_1 \vec{S}_1 \cdot \vec{v}_2 - \frac{3}{64} \vec{S}_1 \cdot \vec{S}_1 \vec{v}_1 \cdot \vec{v}_2 \right) \}$$

$$\left\{ \text{DiagS1S1}[3, 7, 6], \quad \emptyset \right\}$$
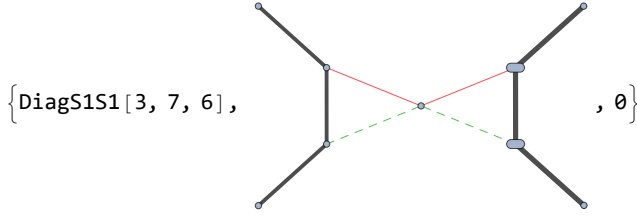

$$\left\{ \text{DiagS1S1}[3, 7, 7], \quad \right\}$$
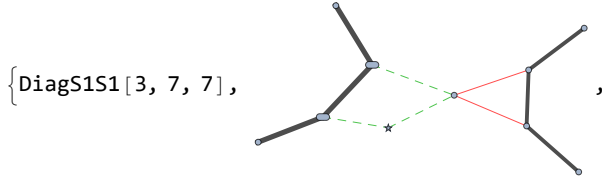

$$\pi^2 G^3 m_2^2 \left\{ \frac{1}{r^5} \left( \frac{945}{128} (\hat{n} \cdot \vec{S}_1)^2 (\hat{n} \cdot \vec{v}_1)^2 - \frac{105}{8} (\hat{n} \cdot \vec{S}_1)^2 \hat{n} \cdot \vec{v}_1 \hat{n} \cdot \vec{v}_2 - \frac{135}{128} \vec{v}_1 \cdot \vec{v}_1 (\hat{n} \cdot \vec{S}_1)^2 + \frac{15}{8} \vec{v}_1 \cdot \vec{v}_2 (\hat{n} \cdot \vec{S}_1)^2 - \right. \right.$$

$$\frac{135}{32} \hat{n} \cdot \vec{S}_1 \hat{n} \cdot \vec{v}_1 \vec{S}_1 \cdot \vec{v}_1 + \frac{15}{4} \hat{n} \cdot \vec{S}_1 \hat{n} \cdot \vec{v}_2 \vec{S}_1 \cdot \vec{v}_1 + \frac{15}{4} \hat{n} \cdot \vec{S}_1 \hat{n} \cdot \vec{v}_1 \vec{S}_1 \cdot \vec{v}_2 - \frac{135}{128} \vec{S}_1 \cdot \vec{S}_1 (\hat{n} \cdot \vec{v}_1)^2 +$$

$$\frac{15}{8} \vec{S}_1 \cdot \vec{S}_1 \hat{n} \cdot \vec{v}_1 \hat{n} \cdot \vec{v}_2 + \frac{27}{64} (\vec{S}_1 \cdot \vec{v}_1)^2 - \frac{3}{4} \vec{S}_1 \cdot \vec{v}_1 \vec{S}_1 \cdot \vec{v}_2 + \frac{27}{128} \vec{S}_1 \cdot \vec{S}_1 \vec{v}_1 \cdot \vec{v}_1 - \frac{3}{8} \vec{S}_1 \cdot \vec{S}_1 \vec{v}_1 \cdot \vec{v}_2 \left. \right) + \frac{1}{r^4}$$

$$\left( -\frac{75}{8} \hat{n} \cdot \vec{S}_1 \hat{n} \cdot \vec{S}_1 \hat{n} \cdot \vec{v}_1 + \frac{15}{8} \vec{S}_1 \cdot \vec{S}_1 \hat{n} \cdot \vec{v}_1 + \frac{75}{8} \hat{n} \cdot \vec{S}_1 \hat{n} \cdot \vec{S}_1 \hat{n} \cdot \vec{v}_2 + \frac{15}{8} \hat{n} \cdot \vec{S}_1 \vec{S}_1 \cdot \vec{v}_1 - \frac{15}{8} \hat{n} \cdot \vec{S}_1 \vec{S}_1 \cdot \vec{v}_2 - \right.$$

$$\left. \frac{15}{8} \vec{S}_1 \cdot \vec{S}_1 \hat{n} \cdot \vec{v}_2 + \frac{15}{8} \hat{n} \cdot \vec{S}_1 \vec{S}_1 \cdot \vec{v}_1 - \frac{15}{8} \hat{n} \cdot \vec{S}_1 \vec{S}_1 \cdot \vec{v}_2 \right) + \frac{\frac{15}{8} (\hat{n} \cdot \vec{S}_1)^2 - \frac{5}{8} \vec{S}_1 \cdot \vec{S}_1}{r^3} \left. \right\}$$

$$\left\{ \text{DiagS1S1}[3, 7, 8], \quad \right\}$$
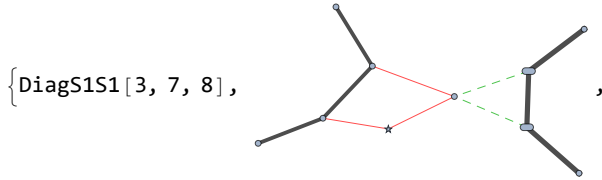

$$\pi^2 G^3 m_2^2 \left\{ \frac{1}{r^5} \left( -\frac{105}{32} (\hat{n} \cdot \vec{S}_1)^2 (\hat{n} \cdot \vec{v}_2)^2 + \frac{105}{16} (\hat{n} \cdot \vec{S}_1)^2 \hat{n} \cdot \vec{v}_1 \hat{n} \cdot \vec{v}_2 - \frac{15}{16} \vec{v}_1 \cdot \vec{v}_2 (\hat{n} \cdot \vec{S}_1)^2 + \frac{15}{32} \vec{v}_2 \cdot \vec{v}_2 (\hat{n} \cdot \vec{S}_1)^2 - \right. \right.$$

$$\frac{15}{8} \hat{n} \cdot \vec{S}_1 \hat{n} \cdot \vec{v}_2 \vec{S}_1 \cdot \vec{v}_1 - \frac{15}{8} \hat{n} \cdot \vec{S}_1 \hat{n} \cdot \vec{v}_1 \vec{S}_1 \cdot \vec{v}_2 + \frac{15}{8} \hat{n} \cdot \vec{S}_1 \hat{n} \cdot \vec{v}_2 \vec{S}_1 \cdot \vec{v}_2 + \frac{15}{32} \vec{S}_1 \cdot \vec{S}_1 (\hat{n} \cdot \vec{v}_2)^2 -$$

$$\frac{15}{16} \vec{S}_1 \cdot \vec{S}_1 \hat{n} \cdot \vec{v}_1 \hat{n} \cdot \vec{v}_2 - \frac{3}{16} (\vec{S}_1 \cdot \vec{v}_2)^2 + \frac{3}{8} \vec{S}_1 \cdot \vec{v}_1 \vec{S}_1 \cdot \vec{v}_2 + \frac{3}{16} \vec{S}_1 \cdot \vec{S}_1 \vec{v}_1 \cdot \vec{v}_2 - \frac{3}{32} \vec{S}_1 \cdot \vec{S}_1 \vec{v}_2 \cdot \vec{v}_2 \left. \right) +$$

$$\frac{-\frac{15}{8} \hat{n} \cdot \vec{S}_1 \hat{n} \cdot \vec{S}_1 \hat{n} \cdot \vec{v}_2 + \frac{3}{8} \vec{S}_1 \cdot \vec{S}_1 \hat{n} \cdot \vec{v}_2 + \frac{3}{8} \hat{n} \cdot \vec{S}_1 \vec{S}_1 \cdot \vec{v}_2 + \frac{3}{8} \hat{n} \cdot \vec{S}_1 \vec{S}_1 \cdot \vec{v}_2}{r^4} \left. \right\}$$

$\{\text{DiagS1S1}[3, 7, 9],$ 
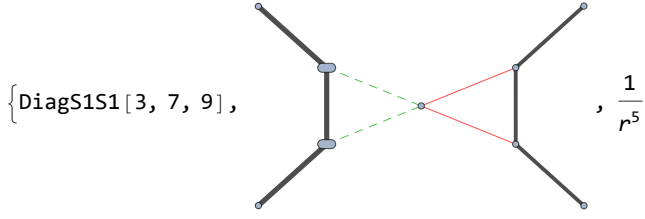
 $, \frac{1}{r^5}$

$$\pi^2 G^3 m_2^2 \left( \frac{105}{128} (\hat{n} \cdot \vec{S}_1)^2 (\hat{n} \cdot \vec{v}_2)^2 - \frac{15}{128} \vec{v}_2 \cdot \vec{v}_2 (\hat{n} \cdot \vec{S}_1)^2 - \frac{15}{32} \hat{n} \cdot \vec{S}_1 \hat{n} \cdot \vec{v}_2 \vec{S}_1 \cdot \vec{v}_2 - \frac{15}{128} \vec{S}_1 \cdot \vec{S}_1 (\hat{n} \cdot \vec{v}_2)^2 + \frac{3}{64} (\vec{S}_1 \cdot \vec{v}_2)^2 + \frac{3}{128} \vec{S}_1 \cdot \vec{S}_1 \vec{v}_2 \cdot \vec{v}_2 \right) \}$$

$\{\text{DiagS1S1}[3, 8, 1],$ 
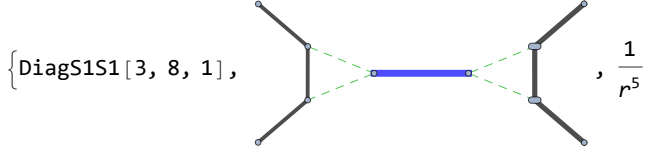
 $, \frac{1}{r^5}$

$$\pi^2 G^3 m_2^2 \left( \frac{315}{128} (\hat{n} \cdot \vec{S}_1)^2 (\hat{n} \cdot \vec{v}_2)^2 - \frac{45}{128} \vec{v}_2 \cdot \vec{v}_2 (\hat{n} \cdot \vec{S}_1)^2 - \frac{45}{32} \hat{n} \cdot \vec{S}_1 \hat{n} \cdot \vec{v}_2 \vec{S}_1 \cdot \vec{v}_2 - \frac{45}{128} \vec{S}_1 \cdot \vec{S}_1 (\hat{n} \cdot \vec{v}_2)^2 + \frac{9}{64} (\vec{S}_1 \cdot \vec{v}_2)^2 + \frac{9}{128} \vec{S}_1 \cdot \vec{S}_1 \vec{v}_2 \cdot \vec{v}_2 \right) \}$$

$\{\text{DiagS1S1}[3, 8, 2],$ 
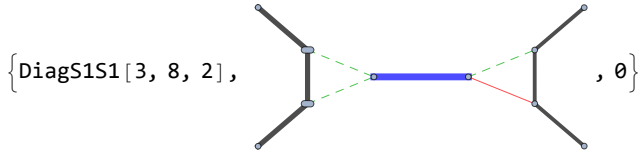
 $, \emptyset\}$

$\{\text{DiagS1S1}[3, 8, 3],$ 
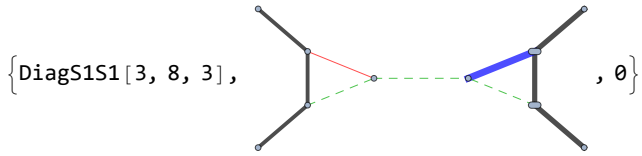
 $, \emptyset\}$

$\{\text{DiagS1S1}[3, 8, 4],$ 
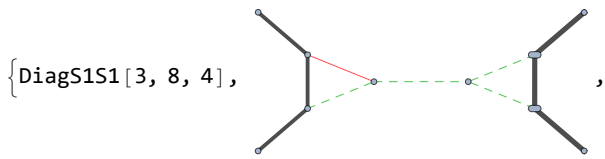
 $,$

$$\pi^2 G^3 m_2^2 \left( \frac{1}{r^5} \left( -\frac{315}{64} (\hat{n} \cdot \vec{S}_1)^2 \hat{n} \cdot \vec{v}_1 \hat{n} \cdot \vec{v}_2 + \frac{45}{64} \vec{v}_1 \cdot \vec{v}_2 (\hat{n} \cdot \vec{S}_1)^2 + \frac{45}{32} \hat{n} \cdot \vec{S}_1 \hat{n} \cdot \vec{v}_2 \vec{S}_1 \cdot \vec{v}_1 + \frac{45}{32} \hat{n} \cdot \vec{S}_1 \hat{n} \cdot \vec{v}_1 \vec{S}_1 \cdot \vec{v}_2 + \frac{45}{64} \vec{S}_1 \cdot \vec{S}_1 \hat{n} \cdot \vec{v}_1 \hat{n} \cdot \vec{v}_2 - \frac{9}{32} \vec{S}_1 \cdot \vec{v}_1 \vec{S}_1 \cdot \vec{v}_2 - \frac{9}{64} \vec{S}_1 \cdot \vec{S}_1 \vec{v}_1 \cdot \vec{v}_2 \right) + \frac{\frac{15}{8} \hat{n} \cdot \vec{S}_1 \hat{n} \cdot \vec{S}_1 \hat{n} \cdot \vec{v}_2 - \frac{3}{8} \vec{S}_1 \cdot \vec{S}_1 \hat{n} \cdot \vec{v}_2 - \frac{3}{8} \hat{n} \cdot \vec{S}_1 \vec{S}_1 \cdot \vec{v}_2 - \frac{3}{8} \hat{n} \cdot \vec{S}_1 \vec{S}_1 \cdot \vec{v}_2}{r^4} \right) \}$$

$\{\text{DiagS1S1}[3, 8, 5],$ 
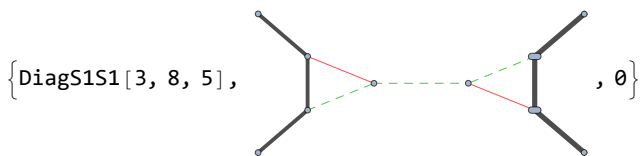
 $, \emptyset\}$

$$\left\{ \text{DiagS1S1}[3, 8, 6], \right. \quad \left. , 0 \right\}$$
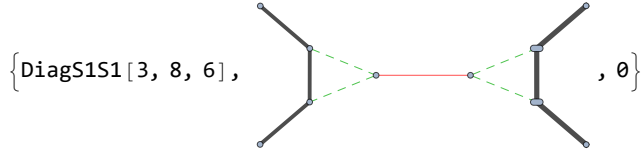

$$\left\{ \text{DiagS1S1}[3, 8, 7], \right. \quad \left. , \frac{1}{r^5} \right\}$$
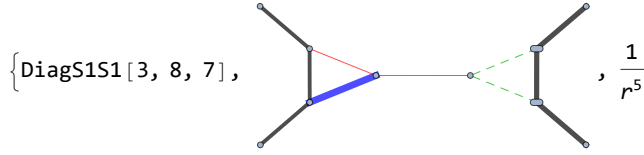

$$\pi^2 G^3 m_2^2 \left( -\frac{105}{16} (\hat{n} \cdot \vec{S}_1)^2 (\hat{n} \cdot \vec{v}_2)^2 + \frac{15}{16} \vec{v}_2 \cdot \vec{v}_2 (\hat{n} \cdot \vec{S}_1)^2 + \frac{15}{4} \hat{n} \cdot \vec{S}_1 \hat{n} \cdot \vec{v}_2 \vec{S}_1 \cdot \vec{v}_2 + \right. \\ \left. \frac{15}{16} \vec{S}_1 \cdot \vec{S}_1 (\hat{n} \cdot \vec{v}_2)^2 - \frac{3}{8} (\vec{S}_1 \cdot \vec{v}_2)^2 - \frac{3}{16} \vec{S}_1 \cdot \vec{S}_1 \vec{v}_2 \cdot \vec{v}_2 \right) \}$$

$$\left\{ \text{DiagS1S1}[3, 8, 8], \right. \quad \left. , 0 \right\}$$
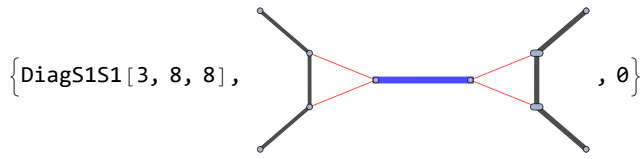

$$\left\{ \text{DiagS1S1}[3, 8, 9], \right. \quad \left. , \frac{1}{r^5} \right\}$$
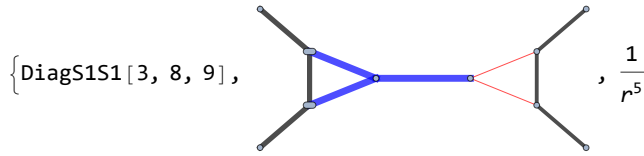

$$\pi^2 G^3 m_2^2 \left( -\frac{315}{256} (\hat{n} \cdot \vec{S}_1)^2 (\hat{n} \cdot \vec{v}_1)^2 + \frac{45}{256} \vec{v}_1 \cdot \vec{v}_1 (\hat{n} \cdot \vec{S}_1)^2 + \frac{45}{64} \hat{n} \cdot \vec{S}_1 \hat{n} \cdot \vec{v}_1 \vec{S}_1 \cdot \vec{v}_1 + \right. \\ \left. \frac{45}{256} \vec{S}_1 \cdot \vec{S}_1 (\hat{n} \cdot \vec{v}_1)^2 - \frac{9}{128} (\vec{S}_1 \cdot \vec{v}_1)^2 - \frac{9}{256} \vec{S}_1 \cdot \vec{S}_1 \vec{v}_1 \cdot \vec{v}_1 \right) \}$$

$$\left\{ \text{DiagS1S1}[3, 8, 10], \right. \quad \left. , \right.$$
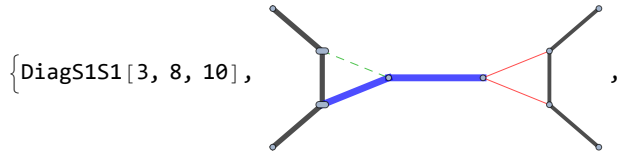

$$\pi^2 G^3 m_2^2 \left( \frac{1}{r^5} \left( \frac{105}{64} (\hat{n} \cdot \vec{S}_1)^2 (\hat{n} \cdot \vec{v}_1)^2 - \frac{15}{64} \vec{v}_1 \cdot \vec{v}_1 (\hat{n} \cdot \vec{S}_1)^2 - \frac{15}{16} \hat{n} \cdot \vec{S}_1 \hat{n} \cdot \vec{v}_1 \vec{S}_1 \cdot \vec{v}_1 - \frac{15}{64} \vec{S}_1 \cdot \vec{S}_1 (\hat{n} \cdot \vec{v}_1)^2 + \right. \right. \\ \left. \left. \frac{3}{32} (\vec{S}_1 \cdot \vec{v}_1)^2 + \frac{3}{64} \vec{S}_1 \cdot \vec{S}_1 \vec{v}_1 \cdot \vec{v}_1 \right) + \frac{-\frac{15}{32} \hat{n} \cdot \vec{S}_1 \hat{n} \cdot \vec{S}_1 \hat{n} \cdot \vec{v}_1 + \frac{3}{32} \vec{S}_1 \cdot \vec{S}_1 \hat{n} \cdot \vec{v}_1 + \frac{3}{32} \hat{n} \cdot \vec{S}_1 \vec{S}_1 \cdot \vec{v}_1 + \frac{3}{32} \hat{n} \cdot \vec{S}_1 \vec{S}_1 \cdot \vec{v}_1}{r^4} \right) \}$$

$$\left\{ \text{DiagS1S1}[3, 8, 11], \right. \quad \left. , 0 \right\}$$
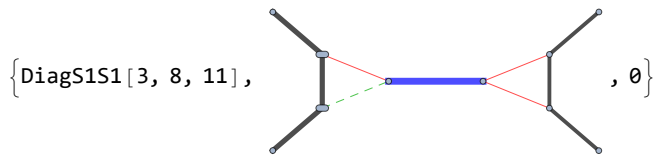

$$\left\{ \text{DiagS1S1}[3, 8, 12], \right. \quad \left. , 0 \right\}$$
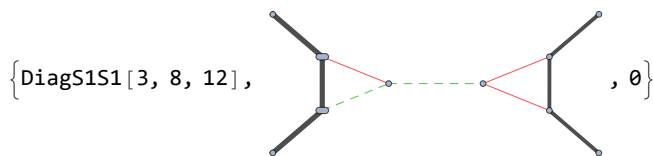

{DiagS1S1[3, 8, 13],

,

$$\pi^2 G^3 m_2^2 \left\{ \frac{1}{r^5} \left( \frac{105}{16} (\hat{n} \cdot \vec{S}_1)^2 (\hat{n} \cdot \vec{v}_2)^2 + \frac{105}{16} (\hat{n} \cdot \vec{S}_1)^2 \hat{n} \cdot \vec{v}_1 \hat{n} \cdot \vec{v}_2 - \frac{15}{16} \vec{v}_1 \cdot \vec{v}_2 (\hat{n} \cdot \vec{S}_1)^2 - \frac{15}{16} \vec{v}_2 \cdot \vec{v}_2 (\hat{n} \cdot \vec{S}_1)^2 - \frac{15}{8} \hat{n} \cdot \vec{S}_1 \hat{n} \cdot \vec{v}_2 \vec{S}_1 \cdot \vec{v}_1 - \frac{15}{8} \hat{n} \cdot \vec{S}_1 \hat{n} \cdot \vec{v}_1 \vec{S}_1 \cdot \vec{v}_2 - \frac{15}{4} \hat{n} \cdot \vec{S}_1 \hat{n} \cdot \vec{v}_2 \vec{S}_1 \cdot \vec{v}_2 - \frac{15}{16} \vec{S}_1 \cdot \vec{S}_1 (\hat{n} \cdot \vec{v}_2)^2 - \frac{15}{16} \vec{S}_1 \cdot \vec{S}_1 \hat{n} \cdot \vec{v}_1 \hat{n} \cdot \vec{v}_2 + \frac{3}{8} (\vec{S}_1 \cdot \vec{v}_2)^2 + \frac{3}{8} \vec{S}_1 \cdot \vec{v}_1 \vec{S}_1 \cdot \vec{v}_2 + \frac{3}{16} \vec{S}_1 \cdot \vec{S}_1 \vec{v}_1 \cdot \vec{v}_2 + \frac{3}{16} \vec{S}_1 \cdot \vec{S}_1 \vec{v}_2 \cdot \vec{v}_2 \right) + \frac{-\frac{15}{8} \hat{n} \cdot \vec{S}_1 \hat{n} \cdot \vec{S}_1 \hat{n} \cdot \vec{v}_2 + \frac{3}{8} \vec{S}_1 \cdot \vec{S}_1 \hat{n} \cdot \vec{v}_2 + \frac{3}{8} \hat{n} \cdot \vec{S}_1 \vec{S}_1 \cdot \vec{v}_2 + \frac{3}{8} \hat{n} \cdot \vec{S}_1 \vec{S}_1 \cdot \vec{v}_2}{r^4} \right\}$$

{DiagS1S1[3, 8, 14],

,

$$\pi^2 G^3 m_2^2 \left\{ \frac{105}{128} (\hat{n} \cdot \vec{S}_1)^2 \hat{n} \cdot \vec{v}_1 \hat{n} \cdot \vec{v}_2 - \frac{15}{128} \vec{v}_1 \cdot \vec{v}_2 (\hat{n} \cdot \vec{S}_1)^2 - \frac{15}{64} \hat{n} \cdot \vec{S}_1 \hat{n} \cdot \vec{v}_2 \vec{S}_1 \cdot \vec{v}_1 - \frac{15}{64} \hat{n} \cdot \vec{S}_1 \hat{n} \cdot \vec{v}_1 \vec{S}_1 \cdot \vec{v}_2 - \frac{15}{128} \vec{S}_1 \cdot \vec{S}_1 \hat{n} \cdot \vec{v}_1 \hat{n} \cdot \vec{v}_2 + \frac{3}{64} \vec{S}_1 \cdot \vec{v}_1 \vec{S}_1 \cdot \vec{v}_2 + \frac{3}{128} \vec{S}_1 \cdot \vec{S}_1 \vec{v}_1 \cdot \vec{v}_2 \right\}$$

{DiagS1S1[3, 8, 15],

,

$$\pi^2 G^3 m_2^2 \left\{ \frac{-\frac{15}{64} \hat{n} \cdot \vec{a}_2 (\hat{n} \cdot \vec{S}_1)^2 + \frac{3}{32} \vec{S}_1 \cdot \vec{a}_2 \hat{n} \cdot \vec{S}_1 + \frac{3}{64} \vec{S}_1 \cdot \vec{S}_1 \hat{n} \cdot \vec{a}_2}{r^4} + \frac{1}{r^5} \left( -\frac{105}{64} (\hat{n} \cdot \vec{S}_1)^2 (\hat{n} \cdot \vec{v}_2)^2 - \frac{105}{1024} (\hat{n} \cdot \vec{S}_1)^2 \hat{n} \cdot \vec{v}_1 \hat{n} \cdot \vec{v}_2 + \frac{15 \vec{v}_1 \cdot \vec{v}_2 (\hat{n} \cdot \vec{S}_1)^2}{1024} + \frac{15}{64} \vec{v}_2 \cdot \vec{v}_2 (\hat{n} \cdot \vec{S}_1)^2 + \frac{15}{512} \hat{n} \cdot \vec{S}_1 \hat{n} \cdot \vec{v}_2 \vec{S}_1 \cdot \vec{v}_1 + \frac{15}{512} \hat{n} \cdot \vec{S}_1 \hat{n} \cdot \vec{v}_1 \vec{S}_1 \cdot \vec{v}_2 + \frac{15}{16} \hat{n} \cdot \vec{S}_1 \hat{n} \cdot \vec{v}_2 \vec{S}_1 \cdot \vec{v}_2 + \frac{15}{64} \vec{S}_1 \cdot \vec{S}_1 (\hat{n} \cdot \vec{v}_2)^2 + \frac{15 \vec{S}_1 \cdot \vec{S}_1 \hat{n} \cdot \vec{v}_1 \hat{n} \cdot \vec{v}_2}{1024} - \frac{3}{32} (\vec{S}_1 \cdot \vec{v}_2)^2 - \frac{3}{512} \vec{S}_1 \cdot \vec{v}_1 \vec{S}_1 \cdot \vec{v}_2 - \frac{3 \vec{S}_1 \cdot \vec{S}_1 \vec{v}_1 \cdot \vec{v}_2}{1024} - \frac{3}{64} \vec{S}_1 \cdot \vec{S}_1 \vec{v}_2 \cdot \vec{v}_2 \right) \right\}$$

{DiagS1S1[3, 8, 16],

,

$$\pi^2 G^3 m_2^2 \left\{ \frac{1}{r^5} \left( \frac{105}{128} (\hat{n} \cdot \vec{S}_1)^2 (\hat{n} \cdot \vec{v}_2)^2 - \frac{105}{16} (\hat{n} \cdot \vec{S}_1)^2 \hat{n} \cdot \vec{v}_1 \hat{n} \cdot \vec{v}_2 + \frac{15}{16} \vec{v}_1 \cdot \vec{v}_2 (\hat{n} \cdot \vec{S}_1)^2 - \frac{15}{128} \vec{v}_2 \cdot \vec{v}_2 (\hat{n} \cdot \vec{S}_1)^2 + \right. \right.$$

$$\left. \begin{aligned} & \frac{15}{8} \hat{n} \cdot \vec{S}_1 \hat{n} \cdot \vec{v}_2 \vec{S}_1 \cdot \vec{v}_1 + \frac{15}{8} \hat{n} \cdot \vec{S}_1 \hat{n} \cdot \vec{v}_1 \vec{S}_1 \cdot \vec{v}_2 - \frac{15}{32} \hat{n} \cdot \vec{S}_1 \hat{n} \cdot \vec{v}_2 \vec{S}_1 \cdot \vec{v}_2 - \frac{15}{128} \vec{S}_1 \cdot \vec{S}_1 (\hat{n} \cdot \vec{v}_2)^2 + \\ & \frac{15}{16} \vec{S}_1 \cdot \vec{S}_1 \hat{n} \cdot \vec{v}_1 \hat{n} \cdot \vec{v}_2 + \frac{3}{64} (\vec{S}_1 \cdot \vec{v}_2)^2 - \frac{3}{8} \vec{S}_1 \cdot \vec{v}_1 \vec{S}_1 \cdot \vec{v}_2 - \frac{3}{16} \vec{S}_1 \cdot \vec{S}_1 \vec{v}_1 \cdot \vec{v}_2 + \frac{3}{128} \vec{S}_1 \cdot \vec{S}_1 \vec{v}_2 \cdot \vec{v}_2 \Big) + \\ & \frac{\frac{15}{8} \hat{n} \cdot \vec{S}_1 \hat{n} \cdot \vec{S}_1 \hat{n} \cdot \vec{v}_2 - \frac{3}{8} \vec{S}_1 \cdot \vec{S}_1 \hat{n} \cdot \vec{v}_2 - \frac{3}{8} \hat{n} \cdot \vec{S}_1 \vec{S}_1 \cdot \vec{v}_2 - \frac{3}{8} \hat{n} \cdot \vec{S}_1 \vec{S}_1 \cdot \vec{v}_2}{r^4} \Big\} \end{aligned}$$

{DiagS1S1[3, 8, 17], 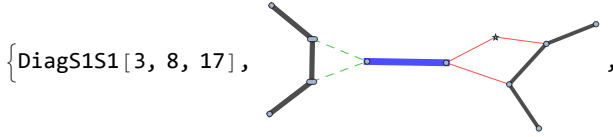 ,

$$\begin{aligned} & \pi^2 G^3 m_2^2 \left( \frac{1}{r^5} \left( -\frac{105 (\hat{n} \cdot \vec{S}_1)^2 (\hat{n} \cdot \vec{v}_2)^2}{2048} - \frac{105}{512} (\hat{n} \cdot \vec{S}_1)^2 \hat{n} \cdot \vec{v}_1 \hat{n} \cdot \vec{v}_2 + \frac{15}{512} \vec{v}_1 \cdot \vec{v}_2 (\hat{n} \cdot \vec{S}_1)^2 + \frac{15 \vec{v}_2 \cdot \vec{v}_2 (\hat{n} \cdot \vec{S}_1)^2}{2048} + \right. \right. \\ & \frac{15}{256} \hat{n} \cdot \vec{S}_1 \hat{n} \cdot \vec{v}_2 \vec{S}_1 \cdot \vec{v}_1 + \frac{15}{256} \hat{n} \cdot \vec{S}_1 \hat{n} \cdot \vec{v}_1 \vec{S}_1 \cdot \vec{v}_2 + \frac{15}{512} \hat{n} \cdot \vec{S}_1 \hat{n} \cdot \vec{v}_2 \vec{S}_1 \cdot \vec{v}_2 + \frac{15 \vec{S}_1 \cdot \vec{S}_1 (\hat{n} \cdot \vec{v}_2)^2}{2048} + \\ & \left. \frac{15}{512} \vec{S}_1 \cdot \vec{S}_1 \hat{n} \cdot \vec{v}_1 \hat{n} \cdot \vec{v}_2 - \frac{3 (\vec{S}_1 \cdot \vec{v}_2)^2}{1024} - \frac{3}{256} \vec{S}_1 \cdot \vec{v}_1 \vec{S}_1 \cdot \vec{v}_2 - \frac{3}{512} \vec{S}_1 \cdot \vec{S}_1 \vec{v}_1 \cdot \vec{v}_2 - \frac{3 \vec{S}_1 \cdot \vec{S}_1 \vec{v}_2 \cdot \vec{v}_2}{2048} \right) + \\ & \left. \frac{\frac{15}{256} \hat{n} \cdot \vec{S}_1 \hat{n} \cdot \vec{S}_1 \hat{n} \cdot \vec{v}_2 - \frac{3}{256} \vec{S}_1 \cdot \vec{S}_1 \hat{n} \cdot \vec{v}_2 - \frac{3}{256} \hat{n} \cdot \vec{S}_1 \vec{S}_1 \cdot \vec{v}_2 - \frac{3}{256} \hat{n} \cdot \vec{S}_1 \vec{S}_1 \cdot \vec{v}_2}{r^4} \right\} \end{aligned}$$

{DiagS1S1[3, 8, 18], 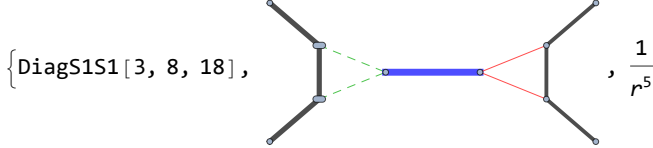 ,  $\frac{1}{r^5}$

$$\begin{aligned} & \pi^2 G^3 m_2^2 \left( -\frac{105}{512} (\hat{n} \cdot \vec{S}_1)^2 (\hat{n} \cdot \vec{v}_2)^2 + \frac{15}{512} \vec{v}_2 \cdot \vec{v}_2 (\hat{n} \cdot \vec{S}_1)^2 + \frac{15}{128} \hat{n} \cdot \vec{S}_1 \hat{n} \cdot \vec{v}_2 \vec{S}_1 \cdot \vec{v}_2 + \right. \\ & \left. \frac{15}{512} \vec{S}_1 \cdot \vec{S}_1 (\hat{n} \cdot \vec{v}_2)^2 - \frac{3}{256} (\vec{S}_1 \cdot \vec{v}_2)^2 - \frac{3}{512} \vec{S}_1 \cdot \vec{S}_1 \vec{v}_2 \cdot \vec{v}_2 \right) \Big\} \end{aligned}$$

{DiagS1S1[3, 8, 19], 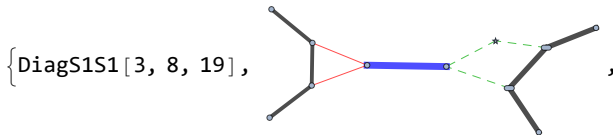 ,

$$\begin{aligned} & \pi^2 G^3 m_2^2 \left( \frac{1}{r^5} \left( \frac{315 (\hat{n} \cdot \vec{S}_1)^2 (\hat{n} \cdot \vec{v}_1)^2}{2048} - \frac{105}{512} (\hat{n} \cdot \vec{S}_1)^2 \hat{n} \cdot \vec{v}_1 \hat{n} \cdot \vec{v}_2 - \frac{45 \vec{v}_1 \cdot \vec{v}_1 (\hat{n} \cdot \vec{S}_1)^2}{2048} + \frac{15}{512} \vec{v}_1 \cdot \vec{v}_2 (\hat{n} \cdot \vec{S}_1)^2 - \right. \right. \\ & \frac{45}{512} \hat{n} \cdot \vec{S}_1 \hat{n} \cdot \vec{v}_1 \vec{S}_1 \cdot \vec{v}_1 + \frac{15}{256} \hat{n} \cdot \vec{S}_1 \hat{n} \cdot \vec{v}_2 \vec{S}_1 \cdot \vec{v}_1 + \frac{15}{256} \hat{n} \cdot \vec{S}_1 \hat{n} \cdot \vec{v}_1 \vec{S}_1 \cdot \vec{v}_2 - \frac{45 \vec{S}_1 \cdot \vec{S}_1 (\hat{n} \cdot \vec{v}_1)^2}{2048} + \\ & \left. \frac{15}{512} \vec{S}_1 \cdot \vec{S}_1 \hat{n} \cdot \vec{v}_1 \hat{n} \cdot \vec{v}_2 + \frac{9 (\vec{S}_1 \cdot \vec{v}_1)^2}{1024} - \frac{3}{256} \vec{S}_1 \cdot \vec{v}_1 \vec{S}_1 \cdot \vec{v}_2 + \frac{9 \vec{S}_1 \cdot \vec{S}_1 \vec{v}_1 \cdot \vec{v}_1}{2048} - \frac{3}{512} \vec{S}_1 \cdot \vec{S}_1 \vec{v}_1 \cdot \vec{v}_2 \right) + \frac{1}{r^4} \\ & \left( -\frac{15}{64} \hat{n} \cdot \vec{S}_1 \hat{n} \cdot \vec{S}_1 \hat{n} \cdot \vec{v}_1 + \frac{3}{64} \vec{S}_1 \cdot \vec{S}_1 \hat{n} \cdot \vec{v}_1 + \frac{15}{64} \hat{n} \cdot \vec{S}_1 \hat{n} \cdot \vec{S}_1 \hat{n} \cdot \vec{v}_2 + \frac{3}{64} \hat{n} \cdot \vec{S}_1 \vec{S}_1 \cdot \vec{v}_1 - \frac{3}{64} \hat{n} \cdot \vec{S}_1 \vec{S}_1 \cdot \vec{v}_2 - \right. \end{aligned}$$

$$\left. \frac{3}{64} \vec{S}_1 \cdot \vec{S}_1 \hat{n} \cdot \vec{v}_2 + \frac{3}{64} \hat{n} \cdot \vec{S}_1 \vec{S}_1 \cdot \vec{v}_1 - \frac{3}{64} \hat{n} \cdot \vec{S}_1 \vec{S}_1 \cdot \vec{v}_2 \right) + \frac{\frac{3}{64} \left( \hat{n} \cdot \vec{S}_1 \right)^2 - \frac{1}{64} \vec{S}_1 \cdot \vec{S}_1}{r^3} \Bigg\}$$

$$\left\{ \text{DiagS1S1} [3, 8, 20], \right.$$
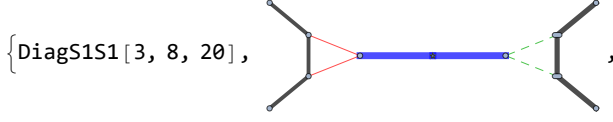

$$,$$

$$\left. \begin{aligned} & \pi^2 G^3 m_2^2 \left\{ \frac{1}{r^5} \left( \frac{105}{512} \left( \hat{n} \cdot \vec{S}_1 \right)^2 \hat{n} \cdot \vec{v}_1 \hat{n} \cdot \vec{v}_2 - \frac{15}{512} \vec{v}_1 \cdot \vec{v}_2 \left( \hat{n} \cdot \vec{S}_1 \right)^2 - \frac{15}{256} \hat{n} \cdot \vec{S}_1 \hat{n} \cdot \vec{v}_2 \vec{S}_1 \cdot \vec{v}_1 - \right. \right. \\ & \frac{15}{256} \hat{n} \cdot \vec{S}_1 \hat{n} \cdot \vec{v}_1 \vec{S}_1 \cdot \vec{v}_2 - \frac{15}{512} \vec{S}_1 \cdot \vec{S}_1 \hat{n} \cdot \vec{v}_1 \hat{n} \cdot \vec{v}_2 + \frac{3}{256} \vec{S}_1 \cdot \vec{v}_1 \vec{S}_1 \cdot \vec{v}_2 + \frac{3}{512} \vec{S}_1 \cdot \vec{S}_1 \vec{v}_1 \cdot \vec{v}_2 \Bigg) + \\ & \left. \left. - \frac{15}{256} \hat{n} \cdot \vec{S}_1 \hat{n} \cdot \vec{S}_1 \hat{n} \cdot \vec{v}_2 + \frac{3}{256} \vec{S}_1 \cdot \vec{S}_1 \hat{n} \cdot \vec{v}_2 + \frac{3}{256} \hat{n} \cdot \vec{S}_1 \vec{S}_1 \cdot \vec{v}_2 + \frac{3}{256} \hat{n} \cdot \vec{S}_1 \vec{S}_1 \cdot \vec{v}_2 \right\} \right. \\ & \left. \frac{1}{r^4} \right\} \end{aligned}$$

$$\left\{ \text{DiagS1S1} [3, 9, 1], \right.$$
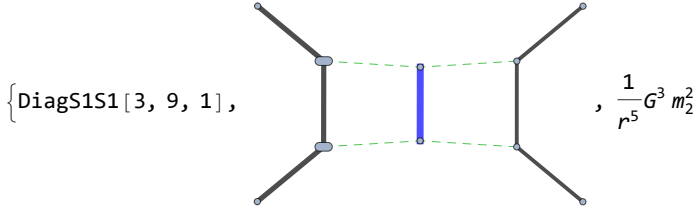

$$, \frac{1}{r^5} G^3 m_2^2$$

$$\left( -2 \left( \hat{n} \times \vec{S}_1 \cdot \vec{v}_2 \right)^2 - 22 \vec{S}_1 \cdot \vec{S}_1 \left( \hat{n} \cdot \vec{v}_2 \right)^2 + 16 \hat{n} \cdot \vec{S}_1 \hat{n} \cdot \vec{v}_2 \vec{S}_1 \cdot \vec{v}_2 - 10 \vec{v}_2 \cdot \vec{v}_2 \left( \hat{n} \cdot \vec{S}_1 \right)^2 - 14 \left( \vec{S}_1 \cdot \vec{v}_2 \right)^2 + 30 \vec{S}_1 \cdot \vec{S}_1 \vec{v}_2 \cdot \vec{v}_2 \right) \Bigg\}$$

$$\left\{ \text{DiagS1S1} [3, 9, 2], \right.$$
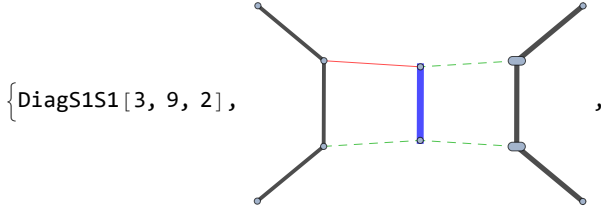

$$,$$

$$\left. \begin{aligned} & G^3 m_2^2 \left\{ \frac{1}{r^5} \left( -36 \left( \hat{n} \times \vec{S}_1 \cdot \vec{v}_2 \right)^2 + 72 \hat{n} \times \vec{S}_1 \cdot \vec{v}_1 \hat{n} \times \vec{S}_1 \cdot \vec{v}_2 - \frac{89}{2} \left( \hat{n} \cdot \vec{S}_1 \right)^2 \left( \hat{n} \cdot \vec{v}_2 \right)^2 + \right. \right. \\ & \frac{141}{2} \left( \hat{n} \cdot \vec{S}_1 \right)^2 \hat{n} \cdot \vec{v}_1 \hat{n} \cdot \vec{v}_2 - \frac{1}{2} \vec{S}_1 \cdot \vec{S}_1 \left( \hat{n} \cdot \vec{v}_2 \right)^2 + \frac{45}{2} \vec{S}_1 \cdot \vec{S}_1 \hat{n} \cdot \vec{v}_1 \hat{n} \cdot \vec{v}_2 - 19 \hat{n} \cdot \vec{S}_1 \hat{n} \cdot \vec{v}_2 \vec{S}_1 \cdot \vec{v}_1 - \\ & 71 \hat{n} \cdot \vec{S}_1 \hat{n} \cdot \vec{v}_1 \vec{S}_1 \cdot \vec{v}_2 + 54 \hat{n} \cdot \vec{S}_1 \hat{n} \cdot \vec{v}_2 \vec{S}_1 \cdot \vec{v}_2 - \frac{19}{2} \vec{v}_1 \cdot \vec{v}_2 \left( \hat{n} \cdot \vec{S}_1 \right)^2 + \frac{71}{2} \vec{v}_2 \cdot \vec{v}_2 \left( \hat{n} \cdot \vec{S}_1 \right)^2 - \\ & 15 \left( \vec{S}_1 \cdot \vec{v}_2 \right)^2 + 27 \vec{S}_1 \cdot \vec{v}_1 \vec{S}_1 \cdot \vec{v}_2 - \frac{33}{2} \vec{S}_1 \cdot \vec{S}_1 \vec{v}_1 \cdot \vec{v}_2 - \frac{35}{2} \vec{S}_1 \cdot \vec{S}_1 \vec{v}_2 \cdot \vec{v}_2 \Bigg) + \frac{1}{r^5} \\ & \pi^2 \left( \frac{105}{32} \left( \hat{n} \cdot \vec{S}_1 \right)^2 \left( \hat{n} \cdot \vec{v}_2 \right)^2 - \frac{105}{32} \left( \hat{n} \cdot \vec{S}_1 \right)^2 \hat{n} \cdot \vec{v}_1 \hat{n} \cdot \vec{v}_2 + \frac{15}{32} \vec{v}_1 \cdot \vec{v}_2 \left( \hat{n} \cdot \vec{S}_1 \right)^2 - \frac{15}{32} \vec{v}_2 \cdot \vec{v}_2 \left( \hat{n} \cdot \vec{S}_1 \right)^2 + \right. \\ & \frac{15}{16} \hat{n} \cdot \vec{S}_1 \hat{n} \cdot \vec{v}_2 \vec{S}_1 \cdot \vec{v}_1 + \frac{15}{16} \hat{n} \cdot \vec{S}_1 \hat{n} \cdot \vec{v}_1 \vec{S}_1 \cdot \vec{v}_2 - \frac{15}{8} \hat{n} \cdot \vec{S}_1 \hat{n} \cdot \vec{v}_2 \vec{S}_1 \cdot \vec{v}_2 - \frac{15}{32} \vec{S}_1 \cdot \vec{S}_1 \left( \hat{n} \cdot \vec{v}_2 \right)^2 + \\ & \frac{15}{32} \vec{S}_1 \cdot \vec{S}_1 \hat{n} \cdot \vec{v}_1 \hat{n} \cdot \vec{v}_2 + \frac{3}{16} \left( \vec{S}_1 \cdot \vec{v}_2 \right)^2 - \frac{3}{16} \vec{S}_1 \cdot \vec{v}_1 \vec{S}_1 \cdot \vec{v}_2 - \frac{3}{32} \vec{S}_1 \cdot \vec{S}_1 \vec{v}_1 \cdot \vec{v}_2 + \frac{3}{32} \vec{S}_1 \cdot \vec{S}_1 \vec{v}_2 \cdot \vec{v}_2 \Bigg) + \\ & \left. \left. - 16 \hat{n} \cdot \vec{S}_1 \hat{n} \cdot \vec{S}_1 \hat{n} \cdot \vec{v}_2 - 8 \vec{S}_1 \cdot \vec{S}_1 \hat{n} \cdot \vec{v}_2 + 28 \hat{n} \cdot \vec{S}_1 \vec{S}_1 \cdot \vec{v}_2 - 4 \hat{n} \cdot \vec{S}_1 \vec{S}_1 \cdot \vec{v}_2 \right\} \right. \\ & \left. \frac{1}{r^4} \right\} \end{aligned}$$

{DiagS1S1[3, 9, 3],

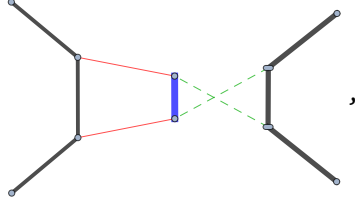

,

$$\begin{aligned}
 G^3 & \left( \frac{12 \vec{S}_1 \cdot \vec{S}_1 - 20 \left( \hat{n} \cdot \vec{S}_1 \right)^2}{r^3} + \frac{1}{r^4} \left( 100 \hat{n} \cdot \vec{S}_1 \hat{n} \cdot \vec{S}_1 \hat{n} \cdot \vec{v}_1 - 36 \vec{S}_1 \cdot \vec{S}_1 \hat{n} \cdot \vec{v}_1 - 118 \hat{n} \cdot \vec{S}_1 \hat{n} \cdot \vec{S}_1 \hat{n} \cdot \vec{v}_2 - \right. \right. \\
 & 28 \hat{n} \cdot \vec{S}_1 \vec{S}_1 \cdot \vec{v}_1 + 24 \hat{n} \cdot \vec{S}_1 \vec{S}_1 \cdot \vec{v}_2 + 38 \hat{n} \cdot \vec{v}_2 \vec{S}_1 \cdot \vec{S}_1 - 12 \hat{n} \cdot \vec{S}_1 \vec{S}_1 \cdot \vec{v}_1 + 20 \hat{n} \cdot \vec{S}_1 \vec{S}_1 \cdot \vec{v}_2 \Big) + \\
 & \frac{1}{r^5} \left( 8 \left( \hat{n} \times \vec{S}_1 \cdot \vec{v}_1 \right)^2 - 22 \hat{n} \times \vec{S}_1 \cdot \vec{v}_2 \hat{n} \times \vec{S}_1 \cdot \vec{v}_1 + 4 \left( \hat{n} \times \vec{S}_1 \cdot \vec{v}_2 \right)^2 - \frac{257}{2} \left( \hat{n} \cdot \vec{S}_1 \right)^2 \left( \hat{n} \cdot \vec{v}_1 \right)^2 - \right. \\
 & \frac{309}{2} \left( \hat{n} \cdot \vec{S}_1 \right)^2 \left( \hat{n} \cdot \vec{v}_2 \right)^2 - 11 \left( \vec{S}_1 \cdot \vec{v}_1 \right)^2 - 11 \left( \vec{S}_1 \cdot \vec{v}_2 \right)^2 + 270 \left( \hat{n} \cdot \vec{S}_1 \right)^2 \hat{n} \cdot \vec{v}_1 \hat{n} \cdot \vec{v}_2 + \frac{39}{2} \left( \hat{n} \cdot \vec{v}_1 \right)^2 \vec{S}_1 \cdot \vec{S}_1 + \\
 & \frac{35}{2} \left( \hat{n} \cdot \vec{v}_2 \right)^2 \vec{S}_1 \cdot \vec{S}_1 - 46 \hat{n} \cdot \vec{v}_1 \hat{n} \cdot \vec{v}_2 \vec{S}_1 \cdot \vec{S}_1 + 86 \hat{n} \cdot \vec{S}_1 \hat{n} \cdot \vec{v}_1 \vec{S}_1 \cdot \vec{v}_1 - 88 \hat{n} \cdot \vec{S}_1 \hat{n} \cdot \vec{v}_2 \vec{S}_1 \cdot \vec{v}_1 - \\
 & 76 \hat{n} \cdot \vec{S}_1 \hat{n} \cdot \vec{v}_1 \vec{S}_1 \cdot \vec{v}_2 + 94 \hat{n} \cdot \vec{S}_1 \hat{n} \cdot \vec{v}_2 \vec{S}_1 \cdot \vec{v}_2 + 18 \vec{S}_1 \cdot \vec{v}_1 \vec{S}_1 \cdot \vec{v}_2 + \frac{15}{2} \left( \hat{n} \cdot \vec{S}_1 \right)^2 \vec{v}_1 \cdot \vec{v}_1 + \\
 & \frac{13}{2} \vec{S}_1 \cdot \vec{S}_1 \vec{v}_1 \cdot \vec{v}_1 - 26 \left( \hat{n} \cdot \vec{S}_1 \right)^2 \vec{v}_1 \cdot \vec{v}_2 - 4 \vec{S}_1 \cdot \vec{S}_1 \vec{v}_1 \cdot \vec{v}_2 + \frac{11}{2} \left( \hat{n} \cdot \vec{S}_1 \right)^2 \vec{v}_2 \cdot \vec{v}_2 + \frac{25}{2} \vec{S}_1 \cdot \vec{S}_1 \vec{v}_2 \cdot \vec{v}_2 \Big) + \\
 & \pi^2 \left( \frac{\frac{3}{2} \left( \hat{n} \cdot \vec{S}_1 \right)^2 - \frac{1}{2} \vec{S}_1 \cdot \vec{S}_1}{r^3} + \frac{1}{r^4} \left( -\frac{15}{2} \hat{n} \cdot \vec{S}_1 \hat{n} \cdot \vec{S}_1 \hat{n} \cdot \vec{v}_1 + \frac{3}{2} \vec{S}_1 \cdot \vec{S}_1 \hat{n} \cdot \vec{v}_1 + \frac{75}{8} \hat{n} \cdot \vec{S}_1 \hat{n} \cdot \vec{S}_1 \hat{n} \cdot \vec{v}_2 + \right. \right. \\
 & \frac{3}{2} \hat{n} \cdot \vec{S}_1 \vec{S}_1 \cdot \vec{v}_1 - \frac{15}{8} \hat{n} \cdot \vec{S}_1 \vec{S}_1 \cdot \vec{v}_2 - \frac{15}{8} \hat{n} \cdot \vec{v}_2 \vec{S}_1 \cdot \vec{S}_1 + \frac{3}{2} \hat{n} \cdot \vec{S}_1 \vec{S}_1 \cdot \vec{v}_1 - \frac{15}{8} \hat{n} \cdot \vec{S}_1 \vec{S}_1 \cdot \vec{v}_2 \Big) + \frac{1}{r^5} \\
 & \left( \frac{315}{32} \left( \hat{n} \cdot \vec{v}_1 \right)^2 \left( \hat{n} \cdot \vec{S}_1 \right)^2 + \frac{315}{32} \left( \hat{n} \cdot \vec{v}_2 \right)^2 \left( \hat{n} \cdot \vec{S}_1 \right)^2 - \frac{315}{16} \hat{n} \cdot \vec{v}_1 \hat{n} \cdot \vec{v}_2 \left( \hat{n} \cdot \vec{S}_1 \right)^2 - \frac{45}{32} \vec{v}_1 \cdot \vec{v}_1 \left( \hat{n} \cdot \vec{S}_1 \right)^2 + \right. \\
 & \frac{45}{16} \vec{v}_1 \cdot \vec{v}_2 \left( \hat{n} \cdot \vec{S}_1 \right)^2 - \frac{45}{32} \vec{v}_2 \cdot \vec{v}_2 \left( \hat{n} \cdot \vec{S}_1 \right)^2 - \frac{45}{8} \hat{n} \cdot \vec{v}_1 \vec{S}_1 \cdot \vec{v}_1 \hat{n} \cdot \vec{S}_1 + \frac{45}{8} \hat{n} \cdot \vec{v}_2 \vec{S}_1 \cdot \vec{v}_1 \hat{n} \cdot \vec{S}_1 + \frac{45}{8} \hat{n} \cdot \vec{v}_1 \vec{S}_1 \cdot \vec{v}_2 \\
 & \hat{n} \cdot \vec{S}_1 - \frac{45}{8} \hat{n} \cdot \vec{v}_2 \vec{S}_1 \cdot \vec{v}_2 \hat{n} \cdot \vec{S}_1 + \frac{9}{16} \left( \vec{S}_1 \cdot \vec{v}_1 \right)^2 + \frac{9}{16} \left( \vec{S}_1 \cdot \vec{v}_2 \right)^2 - \frac{45}{32} \left( \hat{n} \cdot \vec{v}_1 \right)^2 \vec{S}_1 \cdot \vec{S}_1 - \frac{45}{32} \left( \hat{n} \cdot \vec{v}_2 \right)^2 \vec{S}_1 \cdot \vec{S}_1 + \\
 & \left. \left. \frac{45}{16} \hat{n} \cdot \vec{v}_1 \hat{n} \cdot \vec{v}_2 \vec{S}_1 \cdot \vec{S}_1 - \frac{9}{8} \vec{S}_1 \cdot \vec{v}_1 \vec{S}_1 \cdot \vec{v}_2 + \frac{9}{32} \vec{S}_1 \cdot \vec{S}_1 \vec{v}_1 \cdot \vec{v}_1 - \frac{9}{16} \vec{S}_1 \cdot \vec{S}_1 \vec{v}_1 \cdot \vec{v}_2 + \frac{9}{32} \vec{S}_1 \cdot \vec{S}_1 \vec{v}_2 \cdot \vec{v}_2 \right) \right) \Bigg] m_2^2 \Big\}
 \end{aligned}$$

{DiagS1S1[3, 9, 4],

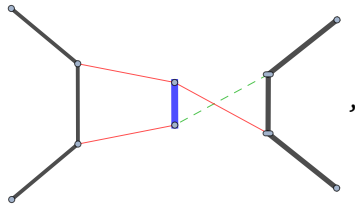

,

$$\begin{aligned}
 G^3 m_2^2 & \left( \frac{1}{r^5} \left( -60 \left( \hat{n} \times \vec{S}_1 \cdot \vec{v}_1 \right)^2 + 44 \hat{n} \times \vec{S}_1 \cdot \vec{v}_2 \hat{n} \times \vec{S}_1 \cdot \vec{v}_1 - 60 \vec{S}_1 \cdot \vec{S}_1 \left( \hat{n} \cdot \vec{v}_1 \right)^2 + \right. \right. \\
 & 42 \vec{S}_1 \cdot \vec{S}_1 \hat{n} \cdot \vec{v}_1 \hat{n} \cdot \vec{v}_2 + 60 \hat{n} \cdot \vec{S}_1 \hat{n} \cdot \vec{v}_1 \vec{S}_1 \cdot \vec{v}_1 - 42 \hat{n} \cdot \vec{S}_1 \hat{n} \cdot \vec{v}_2 \vec{S}_1 \cdot \vec{v}_1 - 24 \left( \vec{S}_1 \cdot \vec{v}_1 \right)^2 +
 \end{aligned}$$

$$14 \vec{S}_1 \cdot \vec{v}_1 \vec{S}_1 \cdot \vec{v}_2 + 24 \vec{S}_1 \cdot \vec{S}_1 \vec{v}_1 \cdot \vec{v}_1 - 14 \vec{S}_1 \cdot \vec{S}_1 \vec{v}_1 \cdot \vec{v}_2 \Big) + \frac{24 \vec{S}_1 \cdot \vec{S}_1 \hat{n} \cdot \vec{v}_1 - 24 \hat{n} \cdot \vec{S}_1 \vec{S}_1 \cdot \vec{v}_1}{r^4} \Bigg\}$$

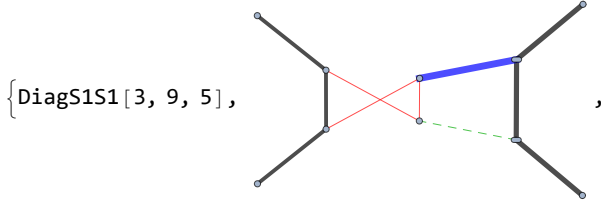

$$G^3 m_2^2 \left( \frac{-\frac{5}{2} \hat{n} \cdot \vec{a}_1 (\hat{n} \cdot \vec{S}_1)^2 + \vec{S}_1 \cdot \vec{a}_1 \hat{n} \cdot \vec{S}_1 + \frac{3}{2} \vec{S}_1 \cdot \vec{S}_1 \hat{n} \cdot \vec{a}_1 - \frac{5}{2} \hat{n} \cdot \vec{S}_1 \hat{n} \cdot \vec{S}_1 \hat{n} \cdot \vec{v}_1 + \frac{3}{2} \vec{S}_1 \cdot \vec{S}_1 \hat{n} \cdot \vec{v}_1 + \hat{n} \cdot \vec{S}_1 \vec{S}_1 \cdot \vec{v}_1}{r^4} + \right. \\ \left. \frac{1}{r^5} \left( -2 (\hat{n} \times \vec{S}_1 \cdot \vec{v}_1)^2 + \hat{n} \times \vec{S}_1 \cdot \vec{v}_2 \hat{n} \times \vec{S}_1 \cdot \vec{v}_1 + \frac{17}{2} (\hat{n} \cdot \vec{S}_1)^2 (\hat{n} \cdot \vec{v}_1)^2 - 7 (\hat{n} \cdot \vec{S}_1)^2 \hat{n} \cdot \vec{v}_1 \hat{n} \cdot \vec{v}_2 - \right. \right. \\ \left. \left. \frac{7}{2} \vec{S}_1 \cdot \vec{S}_1 (\hat{n} \cdot \vec{v}_1)^2 + 7 \vec{S}_1 \cdot \vec{S}_1 \hat{n} \cdot \vec{v}_1 \hat{n} \cdot \vec{v}_2 - 5 \hat{n} \cdot \vec{S}_1 \hat{n} \cdot \vec{v}_1 \vec{S}_1 \cdot \vec{v}_1 - \frac{3}{2} \vec{v}_1 \cdot \vec{v}_1 (\hat{n} \cdot \vec{S}_1)^2 + \right. \right. \\ \left. \left. 2 \vec{v}_1 \cdot \vec{v}_2 (\hat{n} \cdot \vec{S}_1)^2 + \vec{S}_1 \cdot \vec{v}_1 \vec{S}_1 \cdot \vec{v}_2 + \frac{3}{2} \vec{S}_1 \cdot \vec{S}_1 \vec{v}_1 \cdot \vec{v}_1 - 3 \vec{S}_1 \cdot \vec{S}_1 \vec{v}_1 \cdot \vec{v}_2 \right) \right\}$$

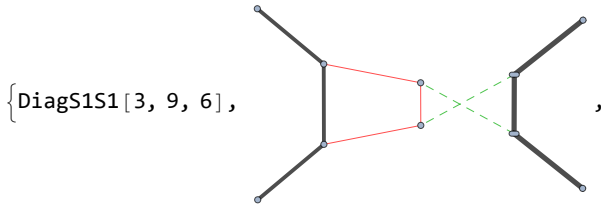

$$G^3 m_2^2 \left( \frac{1}{r^4} \left( \frac{5}{2} \hat{n} \cdot \vec{a}_2 (\hat{n} \cdot \vec{S}_1)^2 - \vec{S}_1 \cdot \vec{a}_2 \hat{n} \cdot \vec{S}_1 - \frac{3}{2} \vec{S}_1 \cdot \vec{S}_1 \hat{n} \cdot \vec{a}_2 + \frac{5}{2} \hat{n} \cdot \vec{S}_1 \hat{n} \cdot \vec{S}_1 \hat{n} \cdot \vec{v}_1 - \right. \right. \\ \left. \left. \hat{n} \cdot \vec{S}_1 \vec{S}_1 \cdot \vec{v}_1 + \hat{n} \cdot \vec{S}_1 \vec{S}_1 \cdot \vec{v}_2 - \frac{3}{2} \vec{S}_1 \cdot \vec{S}_1 \hat{n} \cdot \vec{v}_1 - \hat{n} \cdot \vec{S}_1 \vec{S}_1 \cdot \vec{v}_2 \right) + \frac{1}{r^5} \right. \\ \left( -\frac{1}{2} (\hat{n} \times \vec{S}_1 \cdot \vec{v}_1)^2 + 3 \hat{n} \times \vec{S}_1 \cdot \vec{v}_2 \hat{n} \times \vec{S}_1 \cdot \vec{v}_1 - 2 (\hat{n} \times \vec{S}_1 \cdot \vec{v}_2)^2 - \frac{13}{4} (\hat{n} \cdot \vec{S}_1)^2 (\hat{n} \cdot \vec{v}_1)^2 + \frac{9}{2} (\hat{n} \cdot \vec{S}_1)^2 (\hat{n} \cdot \vec{v}_2)^2 - \right. \\ \left. 2 (\hat{n} \cdot \vec{S}_1)^2 \hat{n} \cdot \vec{v}_1 \hat{n} \cdot \vec{v}_2 + \frac{3}{4} \vec{S}_1 \cdot \vec{S}_1 (\hat{n} \cdot \vec{v}_1)^2 - \frac{9}{2} \vec{S}_1 \cdot \vec{S}_1 (\hat{n} \cdot \vec{v}_2)^2 + 2 \vec{S}_1 \cdot \vec{S}_1 \hat{n} \cdot \vec{v}_1 \hat{n} \cdot \vec{v}_2 + \right. \\ \left. \frac{5}{2} \hat{n} \cdot \vec{S}_1 \hat{n} \cdot \vec{v}_1 \vec{S}_1 \cdot \vec{v}_1 + \frac{1}{4} \vec{v}_1 \cdot \vec{v}_1 (\hat{n} \cdot \vec{S}_1)^2 + \vec{v}_1 \cdot \vec{v}_2 (\hat{n} \cdot \vec{S}_1)^2 - \frac{3}{2} \vec{v}_2 \cdot \vec{v}_2 (\hat{n} \cdot \vec{S}_1)^2 - \frac{1}{2} (\vec{S}_1 \cdot \vec{v}_1)^2 - \right. \\ \left. (\vec{S}_1 \cdot \vec{v}_2)^2 + \vec{S}_1 \cdot \vec{v}_1 \vec{S}_1 \cdot \vec{v}_2 + \frac{1}{4} \vec{S}_1 \cdot \vec{S}_1 \vec{v}_1 \cdot \vec{v}_1 - 2 \vec{S}_1 \cdot \vec{S}_1 \vec{v}_1 \cdot \vec{v}_2 + \frac{5}{2} \vec{S}_1 \cdot \vec{S}_1 \vec{v}_2 \cdot \vec{v}_2 \right) + \frac{\frac{1}{2} \vec{S}_1 \cdot \vec{S}_1 - \frac{1}{2} (\hat{n} \cdot \vec{S}_1)^2}{r^3} \Bigg\}$$

{DiagS1S1[3, 9, 7],

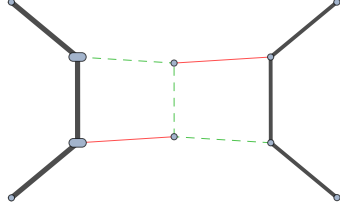

,

$$\frac{G^3 m_2^2 \left( -8 \hat{n} \times \vec{S}_1 \cdot \vec{v}_1 \hat{n} \times \vec{S}_1 \cdot \vec{v}_2 + 8 \vec{S}_1 \cdot \vec{S}_1 \hat{n} \cdot \vec{v}_1 \hat{n} \cdot \vec{v}_2 - 8 \hat{n} \cdot \vec{S}_1 \hat{n} \cdot \vec{v}_2 \vec{S}_1 \cdot \vec{v}_1 \right)}{r^5} \Bigg\}$$

{DiagS1S1[3, 9, 8],

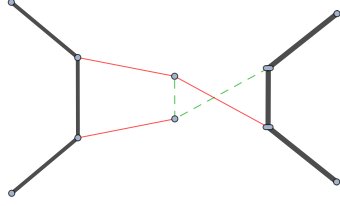

,

$$G^3 m_2^2 \left( \frac{-4 \vec{S}_1 \cdot \vec{a}_1 \hat{n} \cdot \vec{S}_1 + 4 \vec{S}_1 \cdot \vec{S}_1 \hat{n} \cdot \vec{a}_1 + 4 \vec{S}_1 \cdot \vec{S}_1 \hat{n} \cdot \vec{v}_1 - 4 \hat{n} \cdot \vec{S}_1 \vec{S}_1 \cdot \vec{v}_1}{r^4} + \frac{1}{r^5} \left( 8 \left( \hat{n} \times \vec{S}_1 \cdot \vec{v}_1 \right)^2 - 8 \vec{S}_1 \cdot \vec{S}_1 \left( \hat{n} \cdot \vec{v}_1 \right)^2 - \right. \right. \\ \left. \left. 6 \vec{S}_1 \cdot \vec{S}_1 \hat{n} \cdot \vec{v}_1 \hat{n} \cdot \vec{v}_2 + 8 \hat{n} \cdot \vec{S}_1 \hat{n} \cdot \vec{v}_1 \vec{S}_1 \cdot \vec{v}_1 + 6 \hat{n} \cdot \vec{S}_1 \hat{n} \cdot \vec{v}_2 \vec{S}_1 \cdot \vec{v}_1 + 2 \vec{S}_1 \cdot \vec{v}_1 \vec{S}_1 \cdot \vec{v}_2 - 2 \vec{S}_1 \cdot \vec{S}_1 \vec{v}_1 \cdot \vec{v}_2 \right) \right) \Bigg\}$$

{DiagS1S1[3, 9, 9],

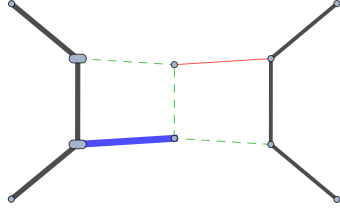

,  $\frac{1}{r^5}$

$$G^3 m_2^2 \left( 10 \hat{n} \times \vec{S}_1 \cdot \vec{v}_1 \hat{n} \times \vec{S}_1 \cdot \vec{v}_2 + 62 \left( \hat{n} \cdot \vec{S}_1 \right)^2 \hat{n} \cdot \vec{v}_1 \hat{n} \cdot \vec{v}_2 - 6 \vec{v}_1 \cdot \vec{v}_2 \left( \hat{n} \cdot \vec{S}_1 \right)^2 - \right. \\ \left. 22 \hat{n} \cdot \vec{S}_1 \hat{n} \cdot \vec{v}_1 \vec{S}_1 \cdot \vec{v}_2 - 40 \vec{S}_1 \cdot \vec{S}_1 \hat{n} \cdot \vec{v}_1 \hat{n} \cdot \vec{v}_2 + 4 \vec{S}_1 \cdot \vec{v}_1 \vec{S}_1 \cdot \vec{v}_2 + 2 \vec{S}_1 \cdot \vec{S}_1 \vec{v}_1 \cdot \vec{v}_2 \right) \Bigg\}$$

{DiagS1S1[3, 9, 10],

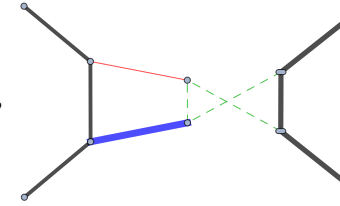

,

$$G^3 m_2^2 \left( \frac{1}{r^5} \left( -2 \left( \hat{n} \times \vec{S}_1 \cdot \vec{v}_2 \right)^2 - 27 \left( \hat{n} \cdot \vec{S}_1 \right)^2 \left( \hat{n} \cdot \vec{v}_2 \right)^2 - 5 \vec{S}_1 \cdot \vec{S}_1 \left( \hat{n} \cdot \vec{v}_2 \right)^2 + 10 \hat{n} \cdot \vec{S}_1 \hat{n} \cdot \vec{v}_2 \vec{S}_1 \cdot \vec{v}_2 + 5 \vec{v}_2 \cdot \vec{v}_2 \left( \hat{n} \cdot \vec{S}_1 \right)^2 - \right. \right. \\ \left. \left. 2 \left( \vec{S}_1 \cdot \vec{v}_2 \right)^2 + 3 \vec{S}_1 \cdot \vec{S}_1 \vec{v}_2 \cdot \vec{v}_2 \right) + \frac{1}{r^5} \pi^2 \left( \frac{735}{64} \left( \hat{n} \cdot \vec{S}_1 \right)^2 \left( \hat{n} \cdot \vec{v}_2 \right)^2 - \frac{105}{64} \vec{v}_2 \cdot \vec{v}_2 \left( \hat{n} \cdot \vec{S}_1 \right)^2 - \right. \right. \\ \left. \left. \frac{105}{16} \hat{n} \cdot \vec{S}_1 \hat{n} \cdot \vec{v}_2 \vec{S}_1 \cdot \vec{v}_2 - \frac{105}{64} \vec{S}_1 \cdot \vec{S}_1 \left( \hat{n} \cdot \vec{v}_2 \right)^2 + \frac{21}{32} \left( \vec{S}_1 \cdot \vec{v}_2 \right)^2 + \frac{21}{64} \vec{S}_1 \cdot \vec{S}_1 \vec{v}_2 \cdot \vec{v}_2 \right) \right) \Bigg\}$$

{DiagS1S1[3, 9, 11],

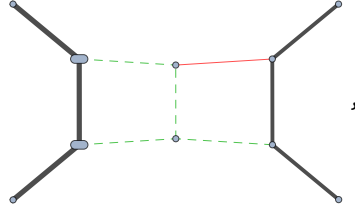

,

$$G^3 \left( \frac{1}{r^4} \left( -10 \hat{n} \cdot \vec{a}_2 \left( \hat{n} \cdot \vec{S}_1 \right)^2 + 8 \hat{n} \cdot \vec{S}_1 \hat{n} \cdot \vec{v}_2 \hat{n} \cdot \vec{S}_1 + 4 \vec{S}_1 \cdot \vec{v}_2 \hat{n} \cdot \vec{S}_1 - 2 \vec{S}_1 \cdot \vec{a}_2 \hat{n} \cdot \vec{S}_1 - 2 \hat{n} \cdot \vec{v}_2 \vec{S}_1 \cdot \vec{S}_1 + 12 \hat{n} \cdot \vec{a}_2 \vec{S}_1 \cdot \vec{S}_1 - \right. \right. \\ \left. \left. 6 \hat{n} \cdot \vec{S}_1 \vec{S}_1 \cdot \vec{v}_2 \right) + \frac{1}{r^5} \left( -14 \left( \hat{n} \times \vec{S}_1 \cdot \vec{v}_2 \right)^2 + \frac{187}{2} \left( \hat{n} \cdot \vec{S}_1 \right)^2 \left( \hat{n} \cdot \vec{v}_2 \right)^2 - 5 \left( \vec{S}_1 \cdot \vec{v}_2 \right)^2 - \frac{47}{2} \left( \hat{n} \cdot \vec{S}_1 \right)^2 \hat{n} \cdot \vec{v}_1 \hat{n} \cdot \vec{v}_2 - \right. \right. \\ \left. \left. \frac{13}{2} \left( \hat{n} \cdot \vec{v}_2 \right)^2 \vec{S}_1 \cdot \vec{S}_1 + \frac{69}{2} \hat{n} \cdot \vec{v}_1 \hat{n} \cdot \vec{v}_2 \vec{S}_1 \cdot \vec{S}_1 - \hat{n} \cdot \vec{S}_1 \hat{n} \cdot \vec{v}_2 \vec{S}_1 \cdot \vec{v}_1 - 11 \hat{n} \cdot \vec{S}_1 \hat{n} \cdot \vec{v}_1 \vec{S}_1 \cdot \vec{v}_2 - 42 \hat{n} \cdot \vec{S}_1 \hat{n} \cdot \vec{v}_2 \vec{S}_1 \cdot \vec{v}_2 + \right. \right. \\ \left. \left. 9 \vec{S}_1 \cdot \vec{v}_1 \vec{S}_1 \cdot \vec{v}_2 + \frac{17}{2} \left( \hat{n} \cdot \vec{S}_1 \right)^2 \vec{v}_1 \cdot \vec{v}_2 - \frac{41}{2} \vec{S}_1 \cdot \vec{S}_1 \vec{v}_1 \cdot \vec{v}_2 - \frac{37}{2} \left( \hat{n} \cdot \vec{S}_1 \right)^2 \vec{v}_2 \cdot \vec{v}_2 + \frac{29}{2} \vec{S}_1 \cdot \vec{S}_1 \vec{v}_2 \cdot \vec{v}_2 \right) + \right. \\ \left. \pi^2 \left( \frac{\frac{15}{8} \hat{n} \cdot \vec{S}_1 \hat{n} \cdot \vec{S}_1 \hat{n} \cdot \vec{v}_2 - \frac{3}{8} \vec{S}_1 \cdot \vec{S}_1 \hat{n} \cdot \vec{v}_2 - \frac{3}{8} \hat{n} \cdot \vec{S}_1 \vec{S}_1 \cdot \vec{v}_2 - \frac{3}{8} \hat{n} \cdot \vec{S}_1 \vec{S}_1 \cdot \vec{v}_2}{r^4} + \frac{1}{r^5} \right. \right. \\ \left. \left( -\frac{525}{32} \left( \hat{n} \cdot \vec{v}_2 \right)^2 \left( \hat{n} \cdot \vec{S}_1 \right)^2 - \frac{105}{16} \hat{n} \cdot \vec{v}_1 \hat{n} \cdot \vec{v}_2 \left( \hat{n} \cdot \vec{S}_1 \right)^2 + \frac{15}{16} \vec{v}_1 \cdot \vec{v}_2 \left( \hat{n} \cdot \vec{S}_1 \right)^2 + \frac{75}{32} \vec{v}_2 \cdot \vec{v}_2 \left( \hat{n} \cdot \vec{S}_1 \right)^2 + \right. \right. \\ \left. \frac{15}{8} \hat{n} \cdot \vec{v}_2 \vec{S}_1 \cdot \vec{v}_1 \hat{n} \cdot \vec{S}_1 + \frac{15}{8} \hat{n} \cdot \vec{v}_1 \vec{S}_1 \cdot \vec{v}_2 \hat{n} \cdot \vec{S}_1 + \frac{75}{8} \hat{n} \cdot \vec{v}_2 \vec{S}_1 \cdot \vec{v}_2 \hat{n} \cdot \vec{S}_1 - \frac{15}{16} \left( \vec{S}_1 \cdot \vec{v}_2 \right)^2 + \right. \\ \left. \left. \frac{75}{32} \left( \hat{n} \cdot \vec{v}_2 \right)^2 \vec{S}_1 \cdot \vec{S}_1 + \frac{15}{16} \hat{n} \cdot \vec{v}_1 \hat{n} \cdot \vec{v}_2 \vec{S}_1 \cdot \vec{S}_1 - \frac{3}{8} \vec{S}_1 \cdot \vec{v}_1 \vec{S}_1 \cdot \vec{v}_2 - \frac{3}{16} \vec{S}_1 \cdot \vec{S}_1 \vec{v}_1 \cdot \vec{v}_2 - \frac{15}{32} \vec{S}_1 \cdot \vec{S}_1 \vec{v}_2 \cdot \vec{v}_2 \right) \right) \left. \right) m_2^2 \}$$

{DiagS1S1[3, 9, 12],

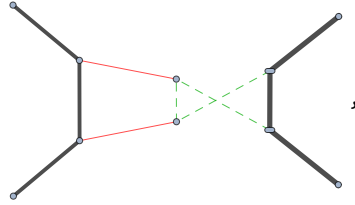

,

$$G^3 m_2^2 \left( \frac{-4 \vec{S}_1 \cdot \vec{a}_1 \hat{n} \cdot \vec{S}_1 + 4 \vec{S}_1 \cdot \vec{S}_1 \hat{n} \cdot \vec{a}_1 + 4 \vec{S}_1 \cdot \vec{S}_1 \hat{n} \cdot \vec{v}_1 - 4 \hat{n} \cdot \vec{S}_1 \vec{S}_1 \cdot \vec{v}_1}{r^4} + \right. \\ \left. \frac{4 \left( \hat{n} \times \vec{S}_1 \cdot \vec{v}_1 \right)^2 - 4 \vec{S}_1 \cdot \vec{S}_1 \left( \hat{n} \cdot \vec{v}_1 \right)^2 + 4 \hat{n} \cdot \vec{S}_1 \hat{n} \cdot \vec{v}_1 \vec{S}_1 \cdot \vec{v}_1}{r^5} \right) \}$$

{DiagS1S1[3, 9, 13],

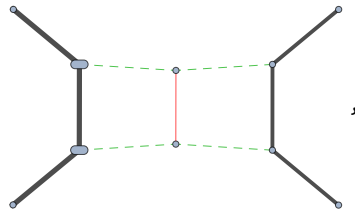

,  $\frac{1}{r^5}$

$$G^3 m_2^2 \left( -52 \left( \hat{n} \cdot \vec{S}_1 \right)^2 \left( \hat{n} \cdot \vec{v}_2 \right)^2 + 4 \vec{v}_2 \cdot \vec{v}_2 \left( \hat{n} \cdot \vec{S}_1 \right)^2 + 56 \hat{n} \cdot \vec{S}_1 \hat{n} \cdot \vec{v}_2 \vec{S}_1 \cdot \vec{v}_2 - \right. \\ \left. 4 \vec{S}_1 \cdot \vec{S}_1 \left( \hat{n} \cdot \vec{v}_2 \right)^2 - 16 \left( \vec{S}_1 \cdot \vec{v}_2 \right)^2 + 12 \vec{S}_1 \cdot \vec{S}_1 \vec{v}_2 \cdot \vec{v}_2 \right) \}$$

{DiagS1S1[3, 9, 14],

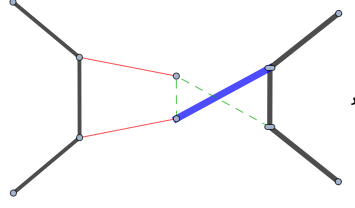

,

$$\begin{aligned}
 & G^3 \left( \frac{-12 \hat{n} \cdot \vec{S}_1 \hat{n} \cdot \vec{S}_1 \hat{n} \cdot \vec{v}_1 + 18 \vec{S}_1 \cdot \vec{S}_1 \hat{n} \cdot \vec{v}_1 - 2 \hat{n} \cdot \vec{S}_1 \vec{S}_1 \cdot \vec{v}_1}{r^4} + \frac{1}{r^5} \right. \\
 & \left( 8 \left( \hat{n} \times \vec{S}_1 \cdot \vec{v}_1 \right)^2 - 6 \hat{n} \times \vec{S}_1 \cdot \vec{v}_2 \hat{n} \times \vec{S}_1 \cdot \vec{v}_1 + \frac{141}{2} \left( \hat{n} \cdot \vec{S}_1 \right)^2 \left( \hat{n} \cdot \vec{v}_1 \right)^2 + \left( \vec{S}_1 \cdot \vec{v}_1 \right)^2 - \frac{193}{2} \left( \hat{n} \cdot \vec{S}_1 \right)^2 \hat{n} \cdot \vec{v}_1 \hat{n} \cdot \vec{v}_2 - \right. \\
 & \frac{119}{2} \left( \hat{n} \cdot \vec{v}_1 \right)^2 \vec{S}_1 \cdot \vec{S}_1 + \frac{139}{2} \hat{n} \cdot \vec{v}_1 \hat{n} \cdot \vec{v}_2 \vec{S}_1 \cdot \vec{S}_1 - 16 \hat{n} \cdot \vec{S}_1 \hat{n} \cdot \vec{v}_1 \vec{S}_1 \cdot \vec{v}_1 - 7 \hat{n} \cdot \vec{S}_1 \hat{n} \cdot \vec{v}_2 \vec{S}_1 \cdot \vec{v}_1 + 39 \hat{n} \cdot \vec{S}_1 \hat{n} \cdot \vec{v}_1 \\
 & \left. \vec{S}_1 \cdot \vec{v}_2 - 3 \vec{S}_1 \cdot \vec{v}_1 \vec{S}_1 \cdot \vec{v}_2 - \frac{19}{2} \left( \hat{n} \cdot \vec{S}_1 \right)^2 \vec{v}_1 \cdot \vec{v}_1 + \frac{19}{2} \vec{S}_1 \cdot \vec{S}_1 \vec{v}_1 \cdot \vec{v}_1 + \frac{23}{2} \left( \hat{n} \cdot \vec{S}_1 \right)^2 \vec{v}_1 \cdot \vec{v}_2 - \frac{19}{2} \vec{S}_1 \cdot \vec{S}_1 \vec{v}_1 \cdot \vec{v}_2 \right) + \\
 & \left. \pi^2 \left( \frac{\frac{15}{8} \hat{n} \cdot \vec{S}_1 \hat{n} \cdot \vec{S}_1 \hat{n} \cdot \vec{v}_1 - \frac{3}{8} \vec{S}_1 \cdot \vec{S}_1 \hat{n} \cdot \vec{v}_1 - \frac{3}{8} \hat{n} \cdot \vec{S}_1 \vec{S}_1 \cdot \vec{v}_1 - \frac{3}{8} \hat{n} \cdot \vec{S}_1 \vec{S}_1 \cdot \vec{v}_1}{r^4} + \frac{1}{r^5} \right. \right. \\
 & \left( -\frac{315}{32} \left( \hat{n} \cdot \vec{v}_1 \right)^2 \left( \hat{n} \cdot \vec{S}_1 \right)^2 + \frac{315}{32} \hat{n} \cdot \vec{v}_1 \hat{n} \cdot \vec{v}_2 \left( \hat{n} \cdot \vec{S}_1 \right)^2 + \frac{45}{32} \vec{v}_1 \cdot \vec{v}_1 \left( \hat{n} \cdot \vec{S}_1 \right)^2 - \frac{45}{32} \vec{v}_1 \cdot \vec{v}_2 \left( \hat{n} \cdot \vec{S}_1 \right)^2 + \right. \\
 & \frac{45}{8} \hat{n} \cdot \vec{v}_1 \vec{S}_1 \cdot \vec{v}_1 \hat{n} \cdot \vec{S}_1 - \frac{45}{16} \hat{n} \cdot \vec{v}_2 \vec{S}_1 \cdot \vec{v}_1 \hat{n} \cdot \vec{S}_1 - \frac{45}{16} \hat{n} \cdot \vec{v}_1 \vec{S}_1 \cdot \vec{v}_2 \hat{n} \cdot \vec{S}_1 - \frac{9}{16} \left( \vec{S}_1 \cdot \vec{v}_1 \right)^2 + \\
 & \left. \left. \frac{45}{32} \left( \hat{n} \cdot \vec{v}_1 \right)^2 \vec{S}_1 \cdot \vec{S}_1 - \frac{45}{32} \hat{n} \cdot \vec{v}_1 \hat{n} \cdot \vec{v}_2 \vec{S}_1 \cdot \vec{S}_1 + \frac{9}{16} \vec{S}_1 \cdot \vec{v}_1 \vec{S}_1 \cdot \vec{v}_2 - \frac{9}{32} \vec{S}_1 \cdot \vec{S}_1 \vec{v}_1 \cdot \vec{v}_1 + \frac{9}{32} \vec{S}_1 \cdot \vec{S}_1 \vec{v}_1 \cdot \vec{v}_2 \right) \right) \left. \right) m_2^2 \}
 \end{aligned}$$

{DiagS1S1[3, 9, 15],

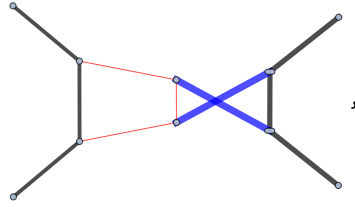

,

$$\begin{aligned}
 & \frac{1}{r^5} G^3 m_2^2 \left( \frac{1}{2} \left( \hat{n} \times \vec{S}_1 \cdot \vec{v}_1 \right)^2 - \frac{3}{4} \left( \hat{n} \cdot \vec{S}_1 \right)^2 \left( \hat{n} \cdot \vec{v}_1 \right)^2 - \frac{7}{4} \vec{S}_1 \cdot \vec{S}_1 \left( \hat{n} \cdot \vec{v}_1 \right)^2 + \right. \\
 & \left. \frac{5}{2} \hat{n} \cdot \vec{S}_1 \hat{n} \cdot \vec{v}_1 \vec{S}_1 \cdot \vec{v}_1 - \frac{1}{4} \vec{v}_1 \cdot \vec{v}_1 \left( \hat{n} \cdot \vec{S}_1 \right)^2 - \frac{1}{2} \left( \vec{S}_1 \cdot \vec{v}_1 \right)^2 + \frac{3}{4} \vec{S}_1 \cdot \vec{S}_1 \vec{v}_1 \cdot \vec{v}_1 \right) \}
 \end{aligned}$$

{DiagS1S1[3, 9, 16],

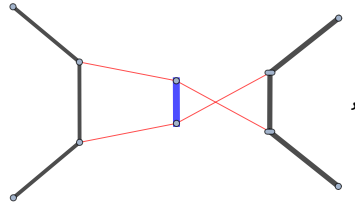

$$, \frac{G^3 m_2^2 \left( 16 \vec{S}_1 \cdot \vec{S}_1 \vec{v}_1 \cdot \vec{v}_1 - 16 \left( \vec{S}_1 \cdot \vec{v}_1 \right)^2 \right)}{r^5} \}$$

{DiagS1S1[3, 9, 17],

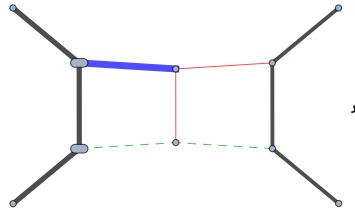

$$, \frac{1}{r^5}$$

$$G^3 m_2^2 \left( 2 \hat{n} \times \vec{S}_1 \cdot \vec{v}_1 \hat{n} \times \vec{S}_1 \cdot \vec{v}_2 - 36 \left( \hat{n} \cdot \vec{S}_1 \right)^2 \hat{n} \cdot \vec{v}_1 \hat{n} \cdot \vec{v}_2 + 4 \vec{v}_1 \cdot \vec{v}_2 \left( \hat{n} \cdot \vec{S}_1 \right)^2 + \right. \\ \left. 10 \hat{n} \cdot \vec{S}_1 \hat{n} \cdot \vec{v}_2 \vec{S}_1 \cdot \vec{v}_1 + 22 \hat{n} \cdot \vec{S}_1 \hat{n} \cdot \vec{v}_1 \vec{S}_1 \cdot \vec{v}_2 + 4 \vec{S}_1 \cdot \vec{S}_1 \hat{n} \cdot \vec{v}_1 \hat{n} \cdot \vec{v}_2 - 6 \vec{S}_1 \cdot \vec{v}_1 \vec{S}_1 \cdot \vec{v}_2 + 2 \vec{S}_1 \cdot \vec{S}_1 \vec{v}_1 \cdot \vec{v}_2 \right) \Big\}$$

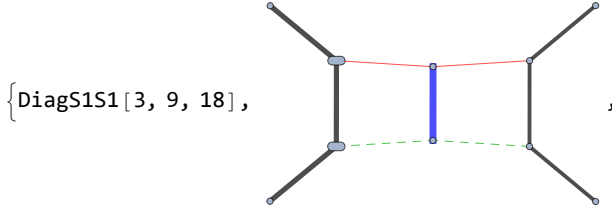

$$G^3 m_2^2 \left( -8 \hat{n} \times \vec{S}_1 \cdot \vec{v}_1 \hat{n} \times \vec{S}_1 \cdot \vec{v}_2 + 28 \vec{S}_1 \cdot \vec{S}_1 \hat{n} \cdot \vec{v}_1 \hat{n} \cdot \vec{v}_2 - 28 \hat{n} \cdot \vec{S}_1 \hat{n} \cdot \vec{v}_2 \vec{S}_1 \cdot \vec{v}_1 + 36 \vec{S}_1 \cdot \vec{v}_1 \vec{S}_1 \cdot \vec{v}_2 - 36 \vec{S}_1 \cdot \vec{S}_1 \vec{v}_1 \cdot \vec{v}_2 \right) \Big\} \\ r^5$$

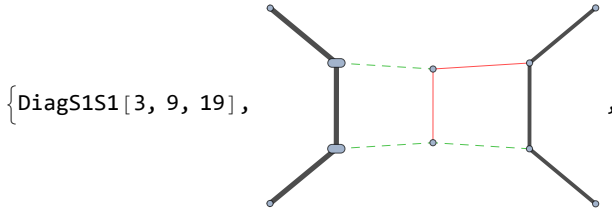

$$G^3 m_2^2 \left( \frac{-10 \hat{n} \cdot \vec{a}_2 \left( \hat{n} \cdot \vec{S}_1 \right)^2 + 6 \vec{S}_1 \cdot \vec{a}_2 \hat{n} \cdot \vec{S}_1 + 4 \vec{S}_1 \cdot \vec{S}_1 \hat{n} \cdot \vec{a}_2 - 10 \hat{n} \cdot \vec{S}_1 \hat{n} \cdot \vec{S}_1 \hat{n} \cdot \vec{v}_2 + 4 \vec{S}_1 \cdot \vec{S}_1 \hat{n} \cdot \vec{v}_2 + 6 \hat{n} \cdot \vec{S}_1 \vec{S}_1 \cdot \vec{v}_2}{r^4} + \frac{1}{r^5} \right. \\ \left( 8 \left( \hat{n} \times \vec{S}_1 \cdot \vec{v}_2 \right)^2 - 10 \hat{n} \times \vec{S}_1 \cdot \vec{v}_1 \hat{n} \times \vec{S}_1 \cdot \vec{v}_2 - 8 \left( \hat{n} \cdot \vec{S}_1 \right)^2 \left( \hat{n} \cdot \vec{v}_2 \right)^2 + 44 \left( \hat{n} \cdot \vec{S}_1 \right)^2 \hat{n} \cdot \vec{v}_1 \hat{n} \cdot \vec{v}_2 + 14 \vec{S}_1 \cdot \vec{S}_1 \left( \hat{n} \cdot \vec{v}_2 \right)^2 - \right. \\ \left. 18 \vec{S}_1 \cdot \vec{S}_1 \hat{n} \cdot \vec{v}_1 \hat{n} \cdot \vec{v}_2 - 10 \hat{n} \cdot \vec{S}_1 \hat{n} \cdot \vec{v}_2 \vec{S}_1 \cdot \vec{v}_1 - 16 \hat{n} \cdot \vec{S}_1 \hat{n} \cdot \vec{v}_1 \vec{S}_1 \cdot \vec{v}_2 - 6 \hat{n} \cdot \vec{S}_1 \hat{n} \cdot \vec{v}_2 \vec{S}_1 \cdot \vec{v}_2 - \right. \\ \left. 8 \vec{v}_1 \cdot \vec{v}_2 \left( \hat{n} \cdot \vec{S}_1 \right)^2 + 4 \vec{v}_2 \cdot \vec{v}_2 \left( \hat{n} \cdot \vec{S}_1 \right)^2 + 6 \left( \vec{S}_1 \cdot \vec{v}_2 \right)^2 + 8 \vec{S}_1 \cdot \vec{S}_1 \vec{v}_1 \cdot \vec{v}_2 - 10 \vec{S}_1 \cdot \vec{S}_1 \vec{v}_2 \cdot \vec{v}_2 \right) \Big\}$$

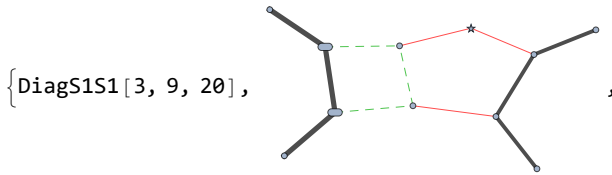

$$G^3 m_2^2 \left( \frac{1}{r^5} \left( 4 \left( \hat{n} \times \vec{S}_1 \cdot \vec{v}_2 \right)^2 + 12 \left( \hat{n} \cdot \vec{S}_1 \right)^2 \left( \hat{n} \cdot \vec{v}_2 \right)^2 - 28 \left( \hat{n} \cdot \vec{S}_1 \right)^2 \hat{n} \cdot \vec{v}_1 \hat{n} \cdot \vec{v}_2 + 2 \vec{S}_1 \cdot \vec{S}_1 \left( \hat{n} \cdot \vec{v}_2 \right)^2 + \right. \right. \\ \left. 10 \vec{S}_1 \cdot \vec{S}_1 \hat{n} \cdot \vec{v}_1 \hat{n} \cdot \vec{v}_2 + 8 \hat{n} \cdot \vec{S}_1 \hat{n} \cdot \vec{v}_2 \vec{S}_1 \cdot \vec{v}_1 - 6 \hat{n} \cdot \vec{S}_1 \hat{n} \cdot \vec{v}_2 \vec{S}_1 \cdot \vec{v}_2 + 4 \vec{v}_1 \cdot \vec{v}_2 \left( \hat{n} \cdot \vec{S}_1 \right)^2 + 2 \vec{v}_2 \cdot \vec{v}_2 \left( \hat{n} \cdot \vec{S}_1 \right)^2 + \right. \\ \left. 2 \left( \vec{S}_1 \cdot \vec{v}_2 \right)^2 - 2 \vec{S}_1 \cdot \vec{S}_1 \vec{v}_1 \cdot \vec{v}_2 - 4 \vec{S}_1 \cdot \vec{S}_1 \vec{v}_2 \cdot \vec{v}_2 \right) + \frac{8 \hat{n} \cdot \vec{S}_1 \hat{n} \cdot \vec{S}_1 \hat{n} \cdot \vec{v}_2 - 4 \vec{S}_1 \cdot \vec{S}_1 \hat{n} \cdot \vec{v}_2}{r^4} + \\ \pi^2 \left( \frac{1}{r^5} \left( \frac{525}{128} \left( \hat{n} \cdot \vec{S}_1 \right)^2 \left( \hat{n} \cdot \vec{v}_2 \right)^2 - \frac{105}{16} \left( \hat{n} \cdot \vec{S}_1 \right)^2 \hat{n} \cdot \vec{v}_1 \hat{n} \cdot \vec{v}_2 + \frac{15}{16} \vec{v}_1 \cdot \vec{v}_2 \left( \hat{n} \cdot \vec{S}_1 \right)^2 - \frac{75}{128} \vec{v}_2 \cdot \vec{v}_2 \left( \hat{n} \cdot \vec{S}_1 \right)^2 + \right. \right. \\ \left. \frac{15}{8} \hat{n} \cdot \vec{S}_1 \hat{n} \cdot \vec{v}_2 \vec{S}_1 \cdot \vec{v}_1 + \frac{15}{8} \hat{n} \cdot \vec{S}_1 \hat{n} \cdot \vec{v}_1 \vec{S}_1 \cdot \vec{v}_2 - \frac{75}{32} \hat{n} \cdot \vec{S}_1 \hat{n} \cdot \vec{v}_2 \vec{S}_1 \cdot \vec{v}_2 - \frac{75}{128} \vec{S}_1 \cdot \vec{S}_1 \left( \hat{n} \cdot \vec{v}_2 \right)^2 + \right. \\ \left. \frac{15}{16} \vec{S}_1 \cdot \vec{S}_1 \hat{n} \cdot \vec{v}_1 \hat{n} \cdot \vec{v}_2 + \frac{15}{64} \left( \vec{S}_1 \cdot \vec{v}_2 \right)^2 - \frac{3}{8} \vec{S}_1 \cdot \vec{v}_1 \vec{S}_1 \cdot \vec{v}_2 - \frac{3}{16} \vec{S}_1 \cdot \vec{S}_1 \vec{v}_1 \cdot \vec{v}_2 + \frac{15}{128} \vec{S}_1 \cdot \vec{S}_1 \vec{v}_2 \cdot \vec{v}_2 \right) + \right.$$

$$\left. \left. \left. \frac{\frac{15}{8} \hat{n} \cdot \vec{S}_1 \hat{n} \cdot \vec{S}_1 \hat{n} \cdot \vec{v}_2 - \frac{3}{8} \vec{S}_1 \cdot \vec{S}_1 \hat{n} \cdot \vec{v}_2 - \frac{3}{8} \hat{n} \cdot \vec{S}_1 \vec{S}_1 \cdot \vec{v}_2 - \frac{3}{8} \hat{n} \cdot \vec{S}_1 \vec{S}_1 \cdot \vec{v}_2}{r^4} \right) \right) \right\}$$

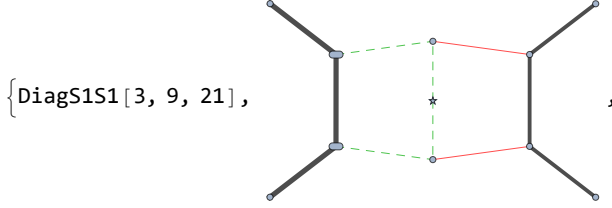

$$\begin{aligned} G^3 & \left( \frac{5 \vec{S}_1 \cdot \vec{S}_1 - 11 \left( \hat{n} \cdot \vec{S}_1 \right)^2}{r^3} + \frac{1}{r^4} \left( 55 \hat{n} \cdot \vec{S}_1 \hat{n} \cdot \vec{S}_1 \hat{n} \cdot \vec{v}_1 - 15 \vec{S}_1 \cdot \vec{S}_1 \hat{n} \cdot \vec{v}_1 - 55 \hat{n} \cdot \vec{S}_1 \hat{n} \cdot \vec{S}_1 \hat{n} \cdot \vec{v}_2 - \right. \right. \\ & 13 \hat{n} \cdot \vec{S}_1 \vec{S}_1 \cdot \vec{v}_1 + 9 \hat{n} \cdot \vec{S}_1 \vec{S}_1 \cdot \vec{v}_2 + 15 \hat{n} \cdot \vec{v}_2 \vec{S}_1 \cdot \vec{S}_1 - 9 \hat{n} \cdot \vec{S}_1 \vec{S}_1 \cdot \vec{v}_1 + 13 \hat{n} \cdot \vec{S}_1 \vec{S}_1 \cdot \vec{v}_2 \Big) + \\ & \frac{1}{r^5} \left( -2 \left( \hat{n} \times \vec{S}_1 \cdot \vec{v}_1 \right)^2 - 10 \hat{n} \times \vec{S}_1 \cdot \vec{v}_2 \hat{n} \times \vec{S}_1 \cdot \vec{v}_1 + 4 \left( \hat{n} \times \vec{S}_1 \cdot \vec{v}_2 \right)^2 - \frac{131}{2} \left( \hat{n} \cdot \vec{S}_1 \right)^2 \left( \hat{n} \cdot \vec{v}_1 \right)^2 - \right. \\ & \frac{143}{2} \left( \hat{n} \cdot \vec{S}_1 \right)^2 \left( \hat{n} \cdot \vec{v}_2 \right)^2 - 5 \left( \vec{S}_1 \cdot \vec{v}_1 \right)^2 + \left( \vec{S}_1 \cdot \vec{v}_2 \right)^2 + \frac{221}{2} \left( \hat{n} \cdot \vec{S}_1 \right)^2 \hat{n} \cdot \vec{v}_1 \hat{n} \cdot \vec{v}_2 + \frac{21}{2} \left( \hat{n} \cdot \vec{v}_1 \right)^2 \vec{S}_1 \cdot \vec{S}_1 + \\ & \frac{37}{2} \left( \hat{n} \cdot \vec{v}_2 \right)^2 \vec{S}_1 \cdot \vec{S}_1 - \frac{63}{2} \hat{n} \cdot \vec{v}_1 \hat{n} \cdot \vec{v}_2 \vec{S}_1 \cdot \vec{S}_1 + 40 \hat{n} \cdot \vec{S}_1 \hat{n} \cdot \vec{v}_1 \vec{S}_1 \cdot \vec{v}_1 - 31 \hat{n} \cdot \vec{S}_1 \hat{n} \cdot \vec{v}_2 \vec{S}_1 \cdot \vec{v}_1 - \\ & 27 \hat{n} \cdot \vec{S}_1 \hat{n} \cdot \vec{v}_1 \vec{S}_1 \cdot \vec{v}_2 + 32 \hat{n} \cdot \vec{S}_1 \hat{n} \cdot \vec{v}_2 \vec{S}_1 \cdot \vec{v}_2 + \vec{S}_1 \cdot \vec{v}_1 \vec{S}_1 \cdot \vec{v}_2 + \frac{17}{2} \left( \hat{n} \cdot \vec{S}_1 \right)^2 \vec{v}_1 \cdot \vec{v}_1 - \\ & \frac{1}{2} \vec{S}_1 \cdot \vec{S}_1 \vec{v}_1 \cdot \vec{v}_1 - \frac{27}{2} \left( \hat{n} \cdot \vec{S}_1 \right)^2 \vec{v}_1 \cdot \vec{v}_2 + \frac{23}{2} \vec{S}_1 \cdot \vec{S}_1 \vec{v}_1 \cdot \vec{v}_2 + \frac{13}{2} \left( \hat{n} \cdot \vec{S}_1 \right)^2 \vec{v}_2 \cdot \vec{v}_2 - \frac{13}{2} \vec{S}_1 \cdot \vec{S}_1 \vec{v}_2 \cdot \vec{v}_2 \Big) + \\ & \pi^2 \left( \frac{\frac{3}{16} \left( \hat{n} \cdot \vec{S}_1 \right)^2 - \frac{1}{16} \vec{S}_1 \cdot \vec{S}_1}{r^3} + \frac{1}{r^4} \left( -\frac{15}{16} \hat{n} \cdot \vec{S}_1 \hat{n} \cdot \vec{S}_1 \hat{n} \cdot \vec{v}_1 + \frac{3}{16} \vec{S}_1 \cdot \vec{S}_1 \hat{n} \cdot \vec{v}_1 + \frac{15}{16} \hat{n} \cdot \vec{S}_1 \hat{n} \cdot \vec{S}_1 \hat{n} \cdot \vec{v}_2 + \right. \right. \\ & \frac{3}{16} \hat{n} \cdot \vec{S}_1 \vec{S}_1 \cdot \vec{v}_1 - \frac{3}{16} \hat{n} \cdot \vec{S}_1 \vec{S}_1 \cdot \vec{v}_2 - \frac{3}{16} \hat{n} \cdot \vec{v}_2 \vec{S}_1 \cdot \vec{S}_1 + \frac{3}{16} \hat{n} \cdot \vec{S}_1 \vec{S}_1 \cdot \vec{v}_1 - \frac{3}{16} \hat{n} \cdot \vec{S}_1 \vec{S}_1 \cdot \vec{v}_2 \Big) + \frac{1}{r^5} \\ & \left( \frac{315}{256} \left( \hat{n} \cdot \vec{v}_1 \right)^2 \left( \hat{n} \cdot \vec{S}_1 \right)^2 + \frac{525}{128} \left( \hat{n} \cdot \vec{v}_2 \right)^2 \left( \hat{n} \cdot \vec{S}_1 \right)^2 - \frac{45}{256} \vec{v}_1 \cdot \vec{v}_1 \left( \hat{n} \cdot \vec{S}_1 \right)^2 - \frac{75}{128} \vec{v}_2 \cdot \vec{v}_2 \left( \hat{n} \cdot \vec{S}_1 \right)^2 - \right. \\ & \frac{45}{64} \hat{n} \cdot \vec{v}_1 \vec{S}_1 \cdot \vec{v}_1 \hat{n} \cdot \vec{S}_1 - \frac{75}{32} \hat{n} \cdot \vec{v}_2 \vec{S}_1 \cdot \vec{v}_2 \hat{n} \cdot \vec{S}_1 + \frac{9}{128} \left( \vec{S}_1 \cdot \vec{v}_1 \right)^2 + \frac{15}{64} \left( \vec{S}_1 \cdot \vec{v}_2 \right)^2 - \\ & \left. \left. \left. \frac{45}{256} \left( \hat{n} \cdot \vec{v}_1 \right)^2 \vec{S}_1 \cdot \vec{S}_1 - \frac{75}{128} \left( \hat{n} \cdot \vec{v}_2 \right)^2 \vec{S}_1 \cdot \vec{S}_1 + \frac{9}{256} \vec{S}_1 \cdot \vec{S}_1 \vec{v}_1 \cdot \vec{v}_1 + \frac{15}{128} \vec{S}_1 \cdot \vec{S}_1 \vec{v}_2 \cdot \vec{v}_2 \right) \right) \right) m_2^2 \Big\} \end{aligned}$$

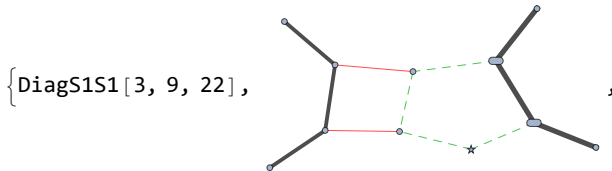

$$\begin{aligned}
& G^3 \left( \frac{3 \frac{1}{S_1} \cdot \frac{1}{S_1} - \left( \hat{n} \cdot \frac{1}{S_1} \right)^2}{r^3} + \frac{1}{r^4} \left( 5 \hat{n} \cdot \frac{1}{S_1} \hat{n} \cdot \vec{S_1} \hat{n} \cdot \vec{v_1} - 9 \vec{S_1} \cdot \frac{1}{S_1} \hat{n} \cdot \vec{v_1} - 5 \hat{n} \cdot \frac{1}{S_1} \hat{n} \cdot \vec{S_1} \hat{n} \cdot \vec{v_2} - \right. \right. \\
& \quad \left. \left. 5 \hat{n} \cdot \vec{S_1} \frac{1}{S_1} \cdot \vec{v_1} + \hat{n} \cdot \vec{S_1} \frac{1}{S_1} \cdot \vec{v_2} + 9 \hat{n} \cdot \vec{v_2} \vec{S_1} \cdot \frac{1}{S_1} + 3 \hat{n} \cdot \frac{1}{S_1} \vec{S_1} \cdot \vec{v_1} + \hat{n} \cdot \frac{1}{S_1} \vec{S_1} \cdot \vec{v_2} \right) + \frac{1}{r^5} \right. \\
& \quad \left( -4 \left( \hat{n} \cdot \vec{S_1} \cdot \vec{v_1} \right)^2 - \frac{9}{2} \left( \hat{n} \cdot \vec{S_1} \right)^2 \left( \hat{n} \cdot \vec{v_1} \right)^2 - 3 \left( \vec{S_1} \cdot \vec{v_1} \right)^2 + 7 \left( \hat{n} \cdot \vec{S_1} \right)^2 \hat{n} \cdot \vec{v_1} \hat{n} \cdot \vec{v_2} - \frac{1}{2} \left( \hat{n} \cdot \vec{v_1} \right)^2 \vec{S_1} \cdot \vec{S_1} - \right. \\
& \quad \left. 5 \hat{n} \cdot \vec{v_1} \hat{n} \cdot \vec{v_2} \vec{S_1} \cdot \vec{S_1} + 10 \hat{n} \cdot \vec{S_1} \hat{n} \cdot \vec{v_1} \vec{S_1} \cdot \vec{v_1} - 10 \hat{n} \cdot \vec{S_1} \hat{n} \cdot \vec{v_2} \vec{S_1} \cdot \vec{v_1} - 2 \hat{n} \cdot \vec{S_1} \hat{n} \cdot \vec{v_1} \vec{S_1} \cdot \vec{v_2} + \right. \\
& \quad \left. 2 \vec{S_1} \cdot \vec{v_1} \vec{S_1} \cdot \vec{v_2} - \frac{1}{2} \left( \hat{n} \cdot \vec{S_1} \right)^2 \vec{v_1} \cdot \vec{v_1} + \frac{5}{2} \vec{S_1} \cdot \vec{S_1} \vec{v_1} \cdot \vec{v_1} - \left( \hat{n} \cdot \vec{S_1} \right)^2 \vec{v_1} \cdot \vec{v_2} + \vec{S_1} \cdot \vec{S_1} \vec{v_1} \cdot \vec{v_2} \right) + \\
& \quad \pi^2 \left( \frac{\frac{15}{16} \frac{1}{S_1} \cdot \frac{1}{S_1} - \frac{45}{16} \left( \hat{n} \cdot \frac{1}{S_1} \right)^2}{r^3} + \frac{1}{r^4} \left( \frac{225}{16} \hat{n} \cdot \frac{1}{S_1} \hat{n} \cdot \vec{S_1} \hat{n} \cdot \vec{v_1} - \frac{45}{16} \vec{S_1} \cdot \frac{1}{S_1} \hat{n} \cdot \vec{v_1} - \frac{225}{16} \hat{n} \cdot \frac{1}{S_1} \hat{n} \cdot \vec{S_1} \hat{n} \cdot \vec{v_2} - \right. \right. \\
& \quad \left. \frac{45}{16} \hat{n} \cdot \vec{S_1} \frac{1}{S_1} \cdot \vec{v_1} + \frac{45}{16} \hat{n} \cdot \vec{S_1} \frac{1}{S_1} \cdot \vec{v_2} + \frac{45}{16} \hat{n} \cdot \vec{v_2} \vec{S_1} \cdot \frac{1}{S_1} - \frac{45}{16} \hat{n} \cdot \frac{1}{S_1} \vec{S_1} \cdot \vec{v_1} + \frac{45}{16} \hat{n} \cdot \frac{1}{S_1} \vec{S_1} \cdot \vec{v_2} \right) + \frac{1}{r^5} \\
& \quad \left( -\frac{2835}{256} \left( \hat{n} \cdot \vec{v_1} \right)^2 \left( \hat{n} \cdot \vec{S_1} \right)^2 + \frac{315}{16} \hat{n} \cdot \vec{v_1} \hat{n} \cdot \vec{v_2} \left( \hat{n} \cdot \vec{S_1} \right)^2 + \frac{405}{256} \vec{v_1} \cdot \vec{v_1} \left( \hat{n} \cdot \vec{S_1} \right)^2 - \frac{45}{16} \vec{v_1} \cdot \vec{v_2} \left( \hat{n} \cdot \vec{S_1} \right)^2 + \right. \\
& \quad \frac{405}{64} \hat{n} \cdot \vec{v_1} \vec{S_1} \cdot \vec{v_1} \hat{n} \cdot \vec{S_1} - \frac{45}{8} \hat{n} \cdot \vec{v_2} \vec{S_1} \cdot \vec{v_1} \hat{n} \cdot \vec{S_1} - \frac{45}{8} \hat{n} \cdot \vec{v_1} \vec{S_1} \cdot \vec{v_2} \hat{n} \cdot \vec{S_1} - \frac{81}{128} \left( \vec{S_1} \cdot \vec{v_1} \right)^2 + \\
& \quad \left. \frac{405}{256} \left( \hat{n} \cdot \vec{v_1} \right)^2 \vec{S_1} \cdot \vec{S_1} - \frac{45}{16} \hat{n} \cdot \vec{v_1} \hat{n} \cdot \vec{v_2} \vec{S_1} \cdot \vec{S_1} + \frac{9}{8} \vec{S_1} \cdot \vec{v_1} \vec{S_1} \cdot \vec{v_2} - \frac{81}{256} \vec{S_1} \cdot \vec{S_1} \vec{v_1} \cdot \vec{v_1} + \frac{9}{16} \vec{S_1} \cdot \vec{S_1} \vec{v_1} \cdot \vec{v_2} \right) \Bigg) \Bigg\} m_2^2 \Bigg\}
\end{aligned}$$
