# Supplementary material for: N$^3$LO Quadratic-in-Spin Interactions for Generic Compact Binaries
Source: arXiv:2209.09235 ancillary file (2023-01-27)
Supplement: Supplementary file 4 [file graphs-S1S2.pdf]

The diagram results are presented in MS-bar scheme.

Definitions :  $G = G_N$ ,  $\epsilon_d = d - 3$ ,  $\hat{n} = \frac{\vec{x}_1 - \vec{x}_2}{r}$ ,  $S_i^2 = \vec{S}_i^2$ ,  $\vec{A} = d^j \vec{A} / dt^j$

Legends :

- $\phi$  propagator
- - - A propagator
- $\sigma$  propagator
- worldlines
- mass coupling
- spin dipole coupling
- spin quadrupole coupling
- ★ time insertion

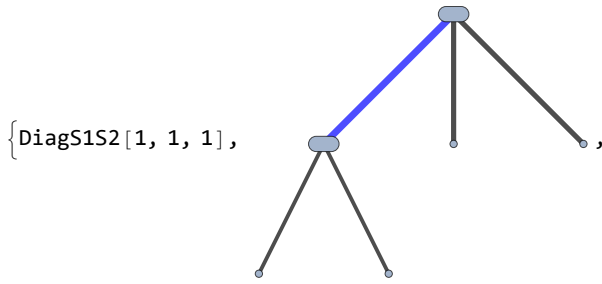

$$\begin{aligned}
 G \left( \frac{1}{r} \left( \frac{9}{4} \vec{S}_1 \cdot \vec{S}_2 (\vec{v}_1 \cdot \vec{v}_2)^2 - \frac{9}{4} \vec{S}_1 \cdot \vec{v}_2 \vec{S}_2 \cdot \vec{v}_1 \vec{v}_1 \cdot \vec{v}_2 + \frac{9}{2} \vec{a}_1 \cdot \vec{v}_2 \vec{S}_1 \cdot \vec{S}_2 \vec{v}_1 \cdot \vec{v}_2 + 5 \vec{a}_1 \cdot \vec{a}_2 \vec{S}_1 \cdot \vec{S}_2 \vec{v}_1 \cdot \vec{v}_2 - \right. \right. \\
 3 \vec{S}_2 \cdot \vec{a}_1 \vec{S}_1 \cdot \vec{v}_2 \vec{v}_1 \cdot \vec{v}_2 - 4 \vec{S}_1 \cdot \vec{a}_2 \vec{S}_2 \cdot \vec{a}_1 \vec{v}_1 \cdot \vec{v}_2 - 3 \vec{S}_1 \cdot \vec{a}_2 \vec{S}_2 \cdot \vec{v}_1 \vec{v}_1 \cdot \vec{v}_2 + \frac{9}{2} \vec{S}_1 \cdot \vec{S}_2 \vec{v}_1 \cdot \vec{a}_2 \vec{v}_1 \cdot \vec{v}_2 - \\
 \frac{9}{4} \vec{S}_1 \times \vec{v}_1 \cdot \vec{v}_2 \vec{S}_2 \times \vec{v}_1 \cdot \vec{v}_2 - 3 \vec{S}_2 \times \vec{v}_1 \cdot \vec{v}_2 \vec{S}_1 \times \vec{a}_1 \cdot \vec{v}_2 - \frac{3}{2} \vec{S}_2 \times \vec{a}_1 \cdot \vec{v}_2 \vec{S}_1 \times \vec{v}_1 \cdot \vec{v}_2 - 2 \vec{S}_1 \times \vec{v}_1 \cdot \vec{v}_2 \vec{S}_2 \times \vec{a}_1 \cdot \vec{a}_2 - \\
 \vec{S}_1 \times \vec{v}_1 \cdot \vec{a}_2 \vec{S}_2 \times \vec{a}_1 \cdot \vec{v}_2 - 3 \vec{S}_1 \times \vec{v}_1 \cdot \vec{v}_2 \vec{S}_2 \times \vec{v}_1 \cdot \vec{a}_2 - 4 \vec{S}_1 \times \vec{a}_1 \cdot \vec{v}_2 \vec{S}_2 \times \vec{v}_1 \cdot \vec{a}_2 - \frac{3}{2} \vec{S}_1 \times \vec{v}_1 \cdot \vec{a}_2 \vec{S}_2 \times \vec{v}_1 \cdot \vec{v}_2 - \\
 2 \vec{S}_1 \times \vec{a}_1 \cdot \vec{a}_2 \vec{S}_2 \times \vec{v}_1 \cdot \vec{v}_2 - 2 \vec{S}_1 \times \vec{v}_1 \cdot \vec{a}_1 \vec{S}_2 \times \vec{v}_2 \cdot \vec{a}_2 - \frac{3}{2} \vec{S}_2 \cdot \vec{v}_1 \vec{a}_1 \cdot \vec{v}_2 \vec{S}_1 \cdot \vec{v}_2 - 2 \vec{a}_1 \cdot \vec{v}_2 \vec{S}_1 \cdot \vec{a}_2 \vec{S}_2 \cdot \vec{v}_1 - \\
 \left. \vec{a}_1 \cdot \vec{a}_2 \vec{S}_1 \cdot \vec{v}_2 \vec{S}_2 \cdot \vec{v}_1 + 4 \vec{a}_1 \cdot \vec{v}_2 \vec{S}_1 \cdot \vec{S}_2 \vec{v}_1 \cdot \vec{a}_2 - 2 \vec{S}_1 \cdot \vec{v}_2 \vec{S}_2 \cdot \vec{a}_1 \vec{v}_1 \cdot \vec{a}_2 - \frac{3}{2} \vec{S}_1 \cdot \vec{v}_2 \vec{S}_2 \cdot \vec{v}_1 \vec{v}_1 \cdot \vec{a}_2 \right) + \\
 \frac{1}{r^2} \left( \frac{3}{4} \hat{n} \cdot \vec{v}_2 \vec{S}_1 \cdot \vec{S}_2 (\vec{v}_1 \cdot \vec{v}_2)^2 - \frac{3}{4} \hat{n} \cdot \vec{v}_1 \vec{S}_1 \cdot \vec{S}_2 (\vec{v}_1 \cdot \vec{v}_2)^2 + \frac{3}{2} \hat{n} \times \vec{S}_2 \cdot \vec{v}_2 \vec{S}_1 \times \vec{v}_1 \cdot \vec{v}_2 \vec{v}_1 \cdot \vec{v}_2 + \right. \\
 \frac{3}{2} \hat{n} \times \vec{S}_1 \cdot \vec{v}_1 \vec{S}_2 \times \vec{v}_1 \cdot \vec{v}_2 \vec{v}_1 \cdot \vec{v}_2 + 2 \hat{n} \times \vec{S}_2 \cdot \vec{v}_2 \vec{S}_1 \times \vec{a}_1 \cdot \vec{v}_2 \vec{v}_1 \cdot \vec{v}_2 - \frac{3}{2} \hat{n} \times \vec{S}_2 \cdot \vec{v}_1 \vec{S}_1 \times \vec{v}_1 \cdot \vec{a}_1 \vec{v}_1 \cdot \vec{v}_2 + \\
 2 \hat{n} \times \vec{S}_1 \cdot \vec{v}_1 \vec{S}_2 \times \vec{v}_1 \cdot \vec{a}_2 \vec{v}_1 \cdot \vec{v}_2 + \frac{3}{2} \hat{n} \times \vec{S}_1 \cdot \vec{v}_2 \vec{S}_2 \times \vec{v}_2 \cdot \vec{a}_2 \vec{v}_1 \cdot \vec{v}_2 + \frac{3}{2} \hat{n} \cdot \vec{v}_2 \vec{a}_1 \cdot \vec{v}_2 \vec{S}_1 \cdot \vec{S}_2 \vec{v}_1 \cdot \vec{v}_2 + \\
 \frac{3}{4} \hat{n} \cdot \vec{v}_1 \vec{S}_2 \cdot \vec{v}_1 \vec{S}_1 \cdot \vec{v}_2 \vec{v}_1 \cdot \vec{v}_2 - \hat{n} \cdot \vec{v}_2 \vec{S}_1 \cdot \vec{v}_2 \vec{S}_2 \cdot \vec{a}_1 \vec{v}_1 \cdot \vec{v}_2 - \frac{3}{4} \hat{n} \cdot \vec{v}_2 \vec{S}_1 \cdot \vec{v}_2 \vec{S}_2 \cdot \vec{v}_1 \vec{v}_1 \cdot \vec{v}_2 + \hat{n} \cdot \vec{v}_1 \vec{S}_1 \cdot \vec{a}_2 \vec{S}_2 \cdot \vec{v}_1 \\
 \vec{v}_1 \cdot \vec{v}_2 - \frac{7}{4} \hat{n} \cdot \vec{v}_1 \vec{S}_1 \cdot \vec{S}_2 \vec{v}_1 \cdot \vec{a}_1 \vec{v}_1 \cdot \vec{v}_2 + \frac{7}{4} \hat{n} \cdot \vec{S}_1 \vec{S}_2 \cdot \vec{v}_1 \vec{v}_1 \cdot \vec{a}_1 \vec{v}_1 \cdot \vec{v}_2 - \frac{3}{2} \hat{n} \cdot \vec{v}_1 \vec{S}_1 \cdot \vec{S}_2 \vec{v}_1 \cdot \vec{a}_2 \vec{v}_1 \cdot \vec{v}_2 - \\
 \frac{7}{8} \hat{n} \cdot \vec{v}_1 \vec{S}_1 \cdot \vec{S}_2 \vec{v}_1 \cdot \vec{v}_1 \vec{v}_1 \cdot \vec{v}_2 - \frac{5}{4} \hat{n} \cdot \vec{a}_1 \vec{S}_1 \cdot \vec{S}_2 \vec{v}_1 \cdot \vec{v}_1 \vec{v}_1 \cdot \vec{v}_2 + \frac{5}{4} \hat{n} \cdot \vec{S}_1 \vec{S}_2 \cdot \vec{a}_1 \vec{v}_1 \cdot \vec{v}_1 \vec{v}_1 \cdot \vec{v}_2 + \\
 \frac{7}{8} \hat{n} \cdot \vec{S}_1 \vec{S}_2 \cdot \vec{v}_1 \vec{v}_1 \cdot \vec{v}_1 \vec{v}_1 \cdot \vec{v}_2 + \frac{7}{4} \hat{n} \cdot \vec{v}_2 \vec{S}_1 \cdot \vec{S}_2 \vec{v}_2 \cdot \vec{a}_2 \vec{v}_1 \cdot \vec{v}_2 - \frac{7}{4} \hat{n} \cdot \vec{S}_2 \vec{S}_1 \cdot \vec{v}_2 \vec{v}_2 \cdot \vec{a}_2 \vec{v}_1 \cdot \vec{v}_2 + \\
 \left. \frac{7}{8} \hat{n} \cdot \vec{v}_2 \vec{S}_1 \cdot \vec{S}_2 \vec{v}_2 \cdot \vec{v}_2 \vec{v}_1 \cdot \vec{v}_2 - \frac{5}{4} \hat{n} \cdot \vec{S}_2 \vec{S}_1 \cdot \vec{a}_2 \vec{v}_2 \cdot \vec{v}_2 \vec{v}_1 \cdot \vec{v}_2 + \frac{5}{4} \hat{n} \cdot \vec{a}_2 \vec{S}_1 \cdot \vec{S}_2 \vec{v}_2 \cdot \vec{v}_2 \vec{v}_1 \cdot \vec{v}_2 - \right.
 \end{aligned}$$

gS1S2[1, 1, 2],

$$G \left( \frac{1}{r} \right) \begin{pmatrix} -4 \vec{S_2} \times \vec{v_1} \cdot \vec{v_2} \vec{S_1} \times \vec{v_1} \cdot \vec{a_1} - 4 \vec{S_2} \times \vec{v_1} \cdot \vec{a_2} \vec{S_1} \times \vec{v_1} \cdot \vec{a_1} + 4 \vec{S_1} \times \vec{v_1} \cdot \vec{v_2} \vec{S_2} \times \vec{v_2} \cdot \vec{a_2} + 4 \vec{S_1} \times \vec{a_1} \cdot \vec{v_2} \vec{S_2} \times \vec{v_2} \cdot \vec{a_2} + \\ 4 \vec{S_2} \cdot \vec{v_1} \vec{S_1} \cdot \vec{v_2} \vec{v_1} \cdot \vec{a_1} + 4 \vec{S_1} \cdot \vec{a_2} \vec{S_2} \cdot \vec{v_1} \vec{v_1} \cdot \vec{a_1} - 4 \vec{S_1} \cdot \vec{S_2} \vec{v_1} \cdot \vec{a_1} \vec{v_1} \cdot \vec{a_2} + 2 \vec{S_1} \cdot \vec{v_2} \vec{S_2} \cdot \vec{v_1} \vec{v_1} \cdot \vec{v_1} - \\ 2 \vec{a_1} \cdot \vec{v_2} \vec{S_1} \cdot \vec{S_2} \vec{v_1} \cdot \vec{v_1} - 2 \vec{a_1} \cdot \vec{a_2} \vec{S_1} \cdot \vec{S_2} \vec{v_1} \cdot \vec{v_1} + 2 \vec{S_2} \cdot \vec{a_1} \vec{S_1} \cdot \vec{v_2} \vec{v_1} \cdot \vec{v_1} + 2 \vec{S_1} \cdot \vec{a_2} \vec{S_2} \cdot \vec{a_1} \vec{v_1} \cdot \vec{v_1} + \\ 2 \vec{S_1} \cdot \vec{a_2} \vec{S_2} \cdot \vec{v_1} \vec{v_1} \cdot \vec{v_1} - 2 \vec{S_1} \cdot \vec{S_2} \vec{v_1} \cdot \vec{a_2} \vec{v_1} \cdot \vec{v_1} - 4 \vec{S_1} \cdot \vec{S_2} \vec{v_1} \cdot \vec{a_1} \vec{v_1} \cdot \vec{v_2} - 2 \vec{S_1} \cdot \vec{S_2} \vec{v_1} \cdot \vec{v_1} \vec{v_1} \cdot \vec{v_2} - \end{pmatrix}$$



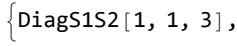

$$G \left( \frac{1}{r^2} \left( -6 \vec{v}_1 \cdot \vec{v}_1 \vec{S}_1 \times \vec{v}_1 \cdot \vec{a}_1 \hat{n} \times \vec{S}_2 \cdot \vec{v}_2 + 2 \vec{v}_1 \cdot \vec{v}_1 \vec{S}_2 \times \vec{v}_2 \cdot \vec{a}_2 \hat{n} \times \vec{S}_1 \cdot \vec{v}_1 - \right. \right. \\ \left. \left. 2 \vec{v}_2 \cdot \vec{v}_2 \vec{S}_1 \times \vec{v}_1 \cdot \vec{a}_1 \hat{n} \times \vec{S}_2 \cdot \vec{v}_2 + 6 \vec{v}_2 \cdot \vec{v}_2 \vec{S}_2 \times \vec{v}_2 \cdot \vec{a}_2 \hat{n} \times \vec{S}_1 \cdot \vec{v}_1 \right) + \frac{4 \vec{S}_1 \times \vec{v}_1 \cdot \vec{a}_1 \vec{S}_2 \times \vec{v}_2 \cdot \vec{a}_2}{r} + \frac{1}{r^3} \right. \\ \left. \left( -\frac{9}{2} (\vec{v}_1 \cdot \vec{v}_1)^2 \hat{n} \times \vec{S}_1 \cdot \vec{v}_1 \hat{n} \times \vec{S}_2 \cdot \vec{v}_2 - 3 \vec{v}_2 \cdot \vec{v}_2 \vec{v}_1 \cdot \vec{v}_1 \hat{n} \times \vec{S}_1 \cdot \vec{v}_1 \hat{n} \times \vec{S}_2 \cdot \vec{v}_2 - \frac{9}{2} (\vec{v}_2 \cdot \vec{v}_2)^2 \hat{n} \times \vec{S}_1 \cdot \vec{v}_1 \hat{n} \times \vec{S}_2 \cdot \vec{v}_2 - \right. \right. \\ \left. \left. \frac{3}{2} (\vec{v}_1 \cdot \vec{v}_1)^2 \vec{S}_1 \cdot \vec{v}_2 \vec{S}_2 \cdot \vec{v}_1 + \frac{3}{2} \vec{S}_1 \cdot \vec{S}_2 \vec{v}_1 \cdot \vec{v}_2 (\vec{v}_1 \cdot \vec{v}_1)^2 - \vec{v}_2 \cdot \vec{v}_2 \vec{v}_1 \cdot \vec{v}_1 \vec{S}_1 \cdot \vec{v}_2 \vec{S}_2 \cdot \vec{v}_1 + \right. \right. \\ \left. \left. \vec{S}_1 \cdot \vec{S}_2 \vec{v}_1 \cdot \vec{v}_2 \vec{v}_2 \cdot \vec{v}_2 \vec{v}_1 \cdot \vec{v}_1 - \frac{3}{2} (\vec{v}_2 \cdot \vec{v}_2)^2 \vec{S}_1 \cdot \vec{v}_2 \vec{S}_2 \cdot \vec{v}_1 + \frac{3}{2} \vec{S}_1 \cdot \vec{S}_2 \vec{v}_1 \cdot \vec{v}_2 (\vec{v}_2 \cdot \vec{v}_2)^2 \right) \right) \Bigg\}$$

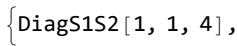

[illegible]













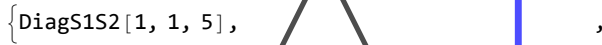

[illegible]



[illegible]



[illegible]











[illegible]

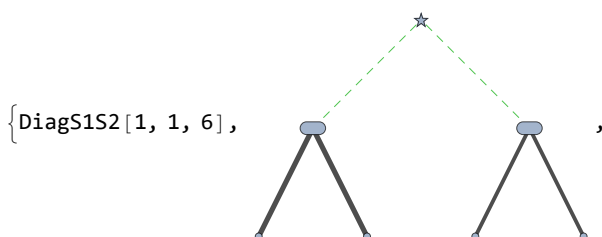

[illegible]

[illegible]











$$\begin{aligned} & \frac{3}{4} \hat{n} \cdot \vec{v}_2 \vec{S}_1 \cdot \vec{S}_2 (\vec{v}_2 \cdot \vec{v}_2)^2 \hat{n} \cdot \vec{v}_1 + \frac{3}{16} \hat{n} \cdot \vec{S}_2 \vec{S}_1 \cdot \vec{v}_2 (\vec{v}_2 \cdot \vec{v}_2)^2 \hat{n} \cdot \vec{v}_1 - \frac{9}{2} \vec{S}_1 \times \vec{v}_1 \cdot \vec{v}_2 \vec{S}_2 \times \vec{v}_1 \cdot \vec{v}_2 \hat{n} \cdot \vec{v}_2 \hat{n} \cdot \vec{v}_1 + \\ & \frac{21}{16} \hat{n} \times \vec{S}_2 \cdot \vec{v}_1 \vec{S}_1 \times \vec{v}_1 \cdot \vec{v}_2 \vec{v}_1 \cdot \vec{v}_1 \hat{n} \cdot \vec{v}_1 + \frac{21}{16} \hat{n} \times \vec{S}_1 \cdot \vec{v}_1 \vec{S}_2 \times \vec{v}_1 \cdot \vec{v}_2 \vec{v}_1 \cdot \vec{v}_1 \hat{n} \cdot \vec{v}_1 - \\ & \frac{105}{16} \hat{n} \times \vec{S}_1 \cdot \vec{v}_1 \hat{n} \times \vec{S}_2 \cdot \vec{v}_1 \hat{n} \cdot \vec{v}_2 \vec{v}_1 \cdot \vec{v}_1 \hat{n} \cdot \vec{v}_1 - \frac{15}{16} \hat{n} \cdot \vec{v}_2 \vec{S}_1 \cdot \vec{v}_1 \vec{S}_2 \cdot \vec{v}_1 \vec{v}_1 \cdot \vec{v}_1 \hat{n} \cdot \vec{v}_1 + \\ & \frac{45}{8} \hat{n} \times \vec{S}_2 \cdot \vec{v}_2 \vec{S}_1 \times \vec{v}_1 \cdot \vec{v}_2 \vec{v}_1 \cdot \vec{v}_2 \hat{n} \cdot \vec{v}_1 - \frac{135}{8} \hat{n} \times \vec{S}_1 \cdot \vec{v}_1 \hat{n} \times \vec{S}_2 \cdot \vec{v}_2 \hat{n} \cdot \vec{v}_2 \vec{v}_1 \cdot \vec{v}_2 \hat{n} \cdot \vec{v}_1 - \\ & \frac{39}{8} \hat{n} \cdot \vec{v}_2 \vec{S}_1 \cdot \vec{v}_2 \vec{S}_2 \cdot \vec{v}_1 \vec{v}_1 \cdot \vec{v}_2 \hat{n} \cdot \vec{v}_1 + \frac{3}{8} \hat{n} \cdot \vec{S}_1 \vec{S}_2 \cdot \vec{v}_1 \vec{v}_1 \cdot \vec{v}_1 \vec{v}_1 \cdot \vec{v}_2 \hat{n} \cdot \vec{v}_1 - \frac{9}{8} \hat{n} \times \vec{S}_1 \cdot \vec{v}_1 \vec{S}_2 \times \vec{v}_1 \cdot \vec{v}_2 \vec{v}_2 \cdot \vec{v}_2 \hat{n} \cdot \vec{v}_1 - \\ & \frac{105}{16} \hat{n} \times \vec{S}_1 \cdot \vec{v}_2 \hat{n} \times \vec{S}_2 \cdot \vec{v}_2 \hat{n} \cdot \vec{v}_2 \vec{v}_2 \cdot \vec{v}_2 \hat{n} \cdot \vec{v}_1 + \frac{15}{16} (\hat{n} \cdot \vec{v}_2)^3 \vec{S}_1 \cdot \vec{S}_2 \vec{v}_2 \cdot \vec{v}_2 \hat{n} \cdot \vec{v}_1 - \\ & \frac{15}{16} \hat{n} \cdot \vec{S}_2 (\hat{n} \cdot \vec{v}_2)^2 \vec{S}_1 \cdot \vec{v}_2 \vec{v}_2 \cdot \vec{v}_2 \hat{n} \cdot \vec{v}_1 - \frac{15}{16} \hat{n} \cdot \vec{v}_2 \vec{S}_1 \cdot \vec{v}_2 \vec{S}_2 \cdot \vec{v}_2 \vec{v}_2 \cdot \vec{v}_2 \hat{n} \cdot \vec{v}_1 - \\ & \frac{11}{8} \vec{S}_1 \cdot \vec{S}_2 (\vec{v}_1 \cdot \vec{v}_2)^3 + \frac{3}{16} \hat{n} \cdot \vec{S}_1 \hat{n} \cdot \vec{v}_2 \vec{S}_2 \cdot \vec{v}_1 (\vec{v}_1 \cdot \vec{v}_1)^2 - \frac{1}{16} \vec{S}_1 \cdot \vec{v}_2 \vec{S}_2 \cdot \vec{v}_1 (\vec{v}_1 \cdot \vec{v}_1)^2 + \\ & \frac{27}{8} \hat{n} \times \vec{S}_1 \cdot \vec{v}_1 \hat{n} \times \vec{S}_2 \cdot \vec{v}_2 (\vec{v}_1 \cdot \vec{v}_2)^2 + \frac{11}{8} \vec{S}_1 \cdot \vec{v}_2 \vec{S}_2 \cdot \vec{v}_1 (\vec{v}_1 \cdot \vec{v}_2)^2 - \frac{1}{16} \vec{S}_1 \cdot \vec{v}_2 \vec{S}_2 \cdot \vec{v}_1 (\vec{v}_2 \cdot \vec{v}_2)^2 - \\ & \frac{1}{4} \vec{S}_1 \cdot \vec{S}_2 \vec{v}_1 \cdot \vec{v}_2 (\vec{v}_2 \cdot \vec{v}_2)^2 + \frac{9}{8} \hat{n} \times \vec{S}_2 \cdot \vec{v}_2 \vec{S}_1 \times \vec{v}_1 \cdot \vec{v}_2 \hat{n} \cdot \vec{v}_2 \vec{v}_1 \cdot \vec{v}_1 - \frac{3}{8} (\hat{n} \cdot \vec{v}_2)^2 \vec{S}_1 \cdot \vec{v}_2 \vec{S}_2 \cdot \vec{v}_1 \vec{v}_1 \cdot \vec{v}_1 - \\ & \frac{1}{4} \vec{S}_1 \cdot \vec{S}_2 (\vec{v}_1 \cdot \vec{v}_1)^2 \vec{v}_1 \cdot \vec{v}_2 + \frac{21}{8} \vec{S}_1 \times \vec{v}_1 \cdot \vec{v}_2 \vec{S}_2 \times \vec{v}_1 \cdot \vec{v}_2 \vec{v}_1 \cdot \vec{v}_2 - \frac{45}{8} \hat{n} \times \vec{S}_1 \cdot \vec{v}_1 \vec{S}_2 \times \vec{v}_1 \cdot \vec{v}_2 \hat{n} \cdot \vec{v}_2 \vec{v}_1 \cdot \vec{v}_2 + \\ & \frac{21}{16} \hat{n} \times \vec{S}_1 \cdot \vec{v}_1 \hat{n} \times \vec{S}_2 \cdot \vec{v}_1 \vec{v}_1 \cdot \vec{v}_1 \vec{v}_1 \cdot \vec{v}_2 + \frac{3}{8} (\hat{n} \cdot \vec{v}_2)^2 \vec{S}_1 \cdot \vec{S}_2 \vec{v}_1 \cdot \vec{v}_1 \vec{v}_1 \cdot \vec{v}_2 + \frac{5}{16} \vec{S}_1 \cdot \vec{v}_1 \vec{S}_2 \cdot \vec{v}_1 \vec{v}_1 \cdot \vec{v}_1 \vec{v}_1 \cdot \vec{v}_2 - \\ & \frac{21}{16} \hat{n} \times \vec{S}_2 \cdot \vec{v}_2 \vec{S}_1 \times \vec{v}_1 \cdot \vec{v}_2 \hat{n} \cdot \vec{v}_2 \vec{v}_2 \cdot \vec{v}_2 - \frac{21}{16} \hat{n} \times \vec{S}_1 \cdot \vec{v}_2 \vec{S}_2 \times \vec{v}_1 \cdot \vec{v}_2 \hat{n} \cdot \vec{v}_2 \vec{v}_2 \cdot \vec{v}_2 + \frac{3}{16} (\hat{n} \cdot \vec{v}_2)^2 \vec{S}_1 \cdot \vec{v}_2 \vec{S}_2 \cdot \vec{v}_1 \vec{v}_2 \cdot \vec{v}_2 + \\ & \left. \left( \frac{1}{8} \vec{S}_1 \cdot \vec{v}_2 \vec{S}_2 \cdot \vec{v}_1 \vec{v}_1 \cdot \vec{v}_1 \vec{v}_2 \cdot \vec{v}_2 + \frac{21}{16} \hat{n} \times \vec{S}_1 \cdot \vec{v}_2 \hat{n} \times \vec{S}_2 \cdot \vec{v}_2 \vec{v}_1 \cdot \vec{v}_2 \vec{v}_2 \cdot \vec{v}_2 - \frac{9}{16} (\hat{n} \cdot \vec{v}_2)^2 \vec{S}_1 \cdot \vec{S}_2 \vec{v}_1 \cdot \vec{v}_2 \vec{v}_2 \cdot \vec{v}_2 + \right. \right. \\ & \left. \left. \frac{3}{8} \hat{n} \cdot \vec{S}_2 \hat{n} \cdot \vec{v}_2 \vec{S}_1 \cdot \vec{v}_2 \vec{v}_1 \cdot \vec{v}_2 \vec{v}_2 \cdot \vec{v}_2 + \frac{5}{16} \vec{S}_1 \cdot \vec{v}_2 \vec{S}_2 \cdot \vec{v}_2 \vec{v}_1 \cdot \vec{v}_2 \vec{v}_2 \cdot \vec{v}_2 - \frac{1}{8} \vec{S}_1 \cdot \vec{S}_2 \vec{v}_1 \cdot \vec{v}_1 \vec{v}_1 \cdot \vec{v}_2 \vec{v}_2 \cdot \vec{v}_2 \right) \right\} \end{aligned}$$

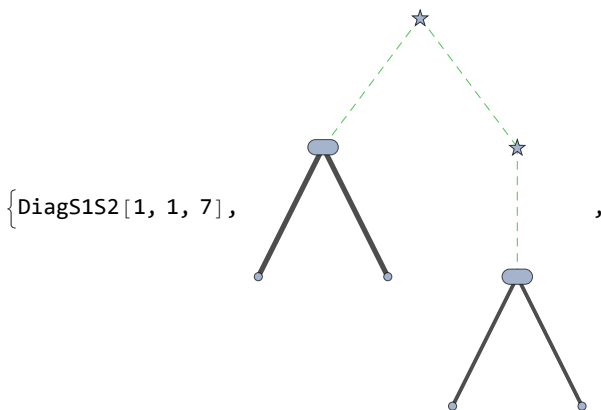

$$G \left( \frac{3}{8} \frac{1}{\vec{S}_1} \cdot \frac{2}{\vec{S}_2} (\hat{n} \cdot \vec{v}_1)^3 - \frac{9}{8} \hat{n} \cdot \vec{v}_2 \frac{1}{\vec{S}_1} \cdot \frac{2}{\vec{S}_2} (\hat{n} \cdot \vec{v}_1)^2 - \frac{9}{16} \hat{n} \cdot \vec{a}_2 \frac{1}{\vec{S}_1} \cdot \frac{2}{\vec{S}_2} (\hat{n} \cdot \vec{v}_1)^2 - \frac{3}{8} \hat{n} \cdot \vec{S}_1 \frac{2}{\vec{S}_2} \cdot \vec{a}_1 (\hat{n} \cdot \vec{v}_1)^2 - \right. \\ \left. \frac{3}{8} \hat{n} \cdot \frac{1}{\vec{S}_1} \frac{2}{\vec{S}_2} \cdot \vec{v}_1 (\hat{n} \cdot \vec{v}_1)^2 + \frac{3}{4} \hat{n} \cdot \frac{1}{\vec{S}_2} \vec{S}_1 \cdot \frac{1}{\vec{a}_2} (\hat{n} \cdot \vec{v}_1)^2 + \frac{1}{4} \hat{n} \cdot \vec{S}_2 \vec{S}_1 \cdot \frac{2}{\vec{a}_2} (\hat{n} \cdot \vec{v}_1)^2 - \frac{3}{4} \hat{n} \cdot \frac{1}{\vec{a}_2} \vec{S}_1 \cdot \frac{1}{\vec{S}_2} (\hat{n} \cdot \vec{v}_1)^2 + \right. \\ \left. \frac{9}{16} \hat{n} \cdot \vec{a}_1 \vec{S}_1 \cdot \frac{2}{\vec{S}_2} (\hat{n} \cdot \vec{v}_1)^2 - \frac{3}{4} \hat{n} \cdot \vec{a}_2 \vec{S}_1 \cdot \frac{2}{\vec{S}_2} (\hat{n} \cdot \vec{v}_1)^2 - \frac{1}{4} \hat{n} \cdot \vec{v}_2 \vec{S}_1 \cdot \frac{3}{\vec{S}_2} (\hat{n} \cdot \vec{v}_1)^2 + \frac{3}{4} \hat{n} \cdot \frac{2}{\vec{S}_2} \vec{S}_1 \cdot \vec{a}_2 (\hat{n} \cdot \vec{v}_1)^2 - \right. \\ \left. \frac{1}{4} \hat{n} \cdot \frac{2}{\vec{a}_2} \vec{S}_1 \cdot \vec{S}_2 (\hat{n} \cdot \vec{v}_1)^2 + \frac{1}{4} \hat{n} \cdot \frac{3}{\vec{S}_2} \vec{S}_1 \cdot \vec{v}_2 (\hat{n} \cdot \vec{v}_1)^2 - \frac{3}{4} \hat{n} \times \vec{S}_1 \cdot \vec{v}_2 \hat{n} \times \frac{1}{\vec{S}_2} \cdot \vec{a}_2 \hat{n} \cdot \vec{v}_1 - \right. \\ \left. \frac{3}{4} \hat{n} \times \vec{S}_1 \cdot \vec{a}_2 \hat{n} \times \frac{1}{\vec{S}_2} \cdot \vec{v}_2 \hat{n} \cdot \vec{v}_1 - \frac{3}{8} \hat{n} \times \vec{S}_1 \cdot \vec{v}_1 \hat{n} \times \frac{2}{\vec{S}_2} \cdot \vec{v}_1 \hat{n} \cdot \vec{v}_1 - \frac{3}{8} \hat{n} \times \vec{S}_1 \cdot \vec{v}_2 \hat{n} \times \frac{2}{\vec{S}_2} \cdot \vec{v}_2 \hat{n} \cdot \vec{v}_1 - \right.$$

[illegible]



[illegible]

























[illegible]



[illegible]

[illegible]

[illegible]



[illegible]









[illegible]





$\{\text{DiagS1S2}[1, 1, 9],$

$$\begin{aligned} & \hat{n} \times \vec{S_1} \cdot \vec{v_1} \vec{S_2} \times \vec{v_1} \cdot \vec{a_2} \vec{v_2} \cdot \vec{v_2} - 3 \hat{n} \times \vec{S_1} \cdot \vec{v_1} \hat{n} \times \vec{S_2} \cdot \vec{v_2} \hat{n} \cdot \vec{v_2} \vec{v_2} \cdot \vec{v_2} - 3 \hat{n} \times \vec{S_1} \cdot \vec{a_1} \hat{n} \times \vec{S_2} \cdot \vec{v_2} \hat{n} \cdot \vec{v_2} \vec{v_2} \cdot \vec{v_2} + \\ & \hat{n} \cdot \vec{v_2} \vec{a_1} \cdot \vec{v_2} \vec{S_1} \cdot \vec{S_2} \vec{v_2} \cdot \vec{v_2} - \hat{n} \cdot \vec{v_2} \vec{S_1} \cdot \vec{v_2} \vec{S_2} \cdot \vec{a_1} \vec{v_2} \cdot \vec{v_2} - \hat{n} \cdot \vec{v_2} \vec{S_1} \cdot \vec{v_2} \vec{S_2} \cdot \vec{v_1} \vec{v_2} \cdot \vec{v_2} + \hat{n} \cdot \vec{v_2} \vec{S_1} \cdot \vec{S_2} \vec{v_1} \cdot \vec{v_2} \vec{v_2} \cdot \vec{v_2} \Bigg) + \\ & \frac{1}{r^3} \left( \vec{S_1} \cdot \vec{S_2} \vec{v_1} \cdot \vec{v_1} (\vec{v_1} \cdot \vec{v_2})^2 + \vec{S_1} \cdot \vec{S_2} \vec{v_2} \cdot \vec{v_2} (\vec{v_1} \cdot \vec{v_2})^2 - 3 \hat{n} \times \vec{S_1} \cdot \vec{v_1} \hat{n} \times \vec{S_2} \cdot \vec{v_2} \vec{v_1} \cdot \vec{v_1} \vec{v_1} \cdot \vec{v_2} - \right. \\ & 3 \hat{n} \cdot \vec{v_1} \hat{n} \cdot \vec{v_2} \vec{S_1} \cdot \vec{S_2} \vec{v_1} \cdot \vec{v_1} \vec{v_1} \cdot \vec{v_2} - \vec{S_1} \cdot \vec{v_2} \vec{S_2} \cdot \vec{v_1} \vec{v_1} \cdot \vec{v_1} \vec{v_1} \cdot \vec{v_2} - 3 \hat{n} \times \vec{S_1} \cdot \vec{v_1} \hat{n} \times \vec{S_2} \cdot \vec{v_2} \vec{v_2} \cdot \vec{v_2} \vec{v_1} \cdot \vec{v_2} - \\ & 3 \hat{n} \cdot \vec{v_1} \hat{n} \cdot \vec{v_2} \vec{S_1} \cdot \vec{S_2} \vec{v_2} \cdot \vec{v_2} \vec{v_1} \cdot \vec{v_2} - \vec{S_1} \cdot \vec{v_2} \vec{S_2} \cdot \vec{v_1} \vec{v_2} \cdot \vec{v_2} \vec{v_1} \cdot \vec{v_2} - \vec{S_1} \times \vec{v_1} \cdot \vec{v_2} \vec{S_2} \times \vec{v_1} \cdot \vec{v_2} \vec{v_1} \cdot \vec{v_1} - \\ & 3 \hat{n} \times \vec{S_2} \cdot \vec{v_2} \vec{S_1} \times \vec{v_1} \cdot \vec{v_2} \hat{n} \cdot \vec{v_1} \vec{v_1} \cdot \vec{v_1} + 3 \hat{n} \times \vec{S_1} \cdot \vec{v_1} \vec{S_2} \times \vec{v_1} \cdot \vec{v_2} \hat{n} \cdot \vec{v_2} \vec{v_1} \cdot \vec{v_1} + \\ & 15 \hat{n} \times \vec{S_1} \cdot \vec{v_1} \hat{n} \times \vec{S_2} \cdot \vec{v_2} \hat{n} \cdot \vec{v_1} \hat{n} \cdot \vec{v_2} \vec{v_1} \cdot \vec{v_1} + 3 \hat{n} \cdot \vec{v_1} \hat{n} \cdot \vec{v_2} \vec{S_1} \cdot \vec{v_2} \vec{S_2} \cdot \vec{v_1} \vec{v_1} \cdot \vec{v_1} - \\ & \vec{S_1} \times \vec{v_1} \cdot \vec{v_2} \vec{S_2} \times \vec{v_1} \cdot \vec{v_2} \vec{v_2} \cdot \vec{v_2} - 3 \hat{n} \times \vec{S_2} \cdot \vec{v_2} \vec{S_1} \times \vec{v_1} \cdot \vec{v_2} \hat{n} \cdot \vec{v_1} \vec{v_2} \cdot \vec{v_2} + 3 \hat{n} \times \vec{S_1} \cdot \vec{v_1} \vec{S_2} \times \vec{v_1} \cdot \vec{v_2} \hat{n} \cdot \vec{v_2} \vec{v_2} \cdot \vec{v_2} + \\ & \left. 15 \hat{n} \times \vec{S_1} \cdot \vec{v_1} \hat{n} \times \vec{S_2} \cdot \vec{v_2} \hat{n} \cdot \vec{v_1} \hat{n} \cdot \vec{v_2} \vec{v_2} \cdot \vec{v_2} + 3 \hat{n} \cdot \vec{v_1} \hat{n} \cdot \vec{v_2} \vec{S_1} \cdot \vec{v_2} \vec{S_2} \cdot \vec{v_1} \vec{v_2} \cdot \vec{v_2} \right) \Bigg\} \end{aligned}$$

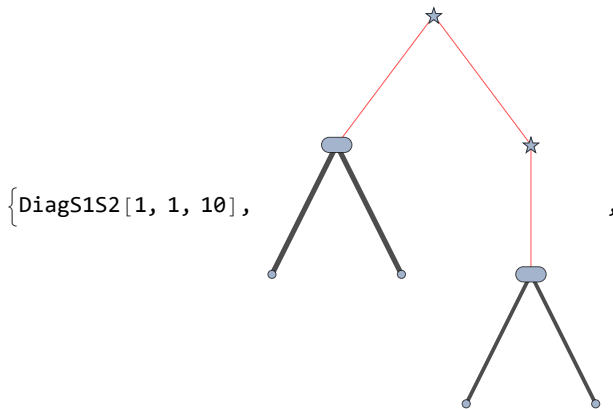

[illegible]





$$\{\text{DiagS1S2}[2, 1, 1],$$

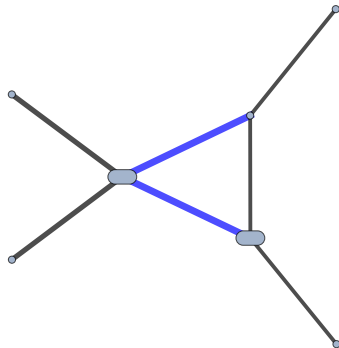



$$G^2 m_2 \left\{ \frac{-2 \vec{S}_1 \times \vec{v}_2 \cdot \vec{a}_2 \hat{n} \times \vec{S}_2 \cdot \vec{v}_2 - \vec{S}_1 \cdot \vec{S}_2 \vec{v}_2 \cdot \vec{v}_2 \hat{n} \cdot \vec{a}_2 + \vec{v}_2 \cdot \vec{v}_2 \vec{S}_2 \cdot \vec{a}_2 \hat{n} \cdot \vec{S}_1 - \vec{v}_2 \cdot \vec{v}_2 \hat{n} \cdot \vec{S}_1 \vec{S}_2 \cdot \vec{v}_2 + \vec{S}_1 \cdot \vec{S}_2 \vec{v}_2 \cdot \vec{v}_2 \hat{n} \cdot \vec{v}_2}{r^3} + \right.$$

$$\frac{1}{r^4} \left( -12 \hat{n} \cdot \vec{v}_2 \vec{S}_1 \times \vec{v}_1 \cdot \vec{v}_2 \hat{n} \times \vec{S}_2 \cdot \vec{v}_2 - 12 \vec{v}_1 \cdot \vec{v}_2 \hat{n} \times \vec{S}_1 \cdot \vec{v}_2 \hat{n} \times \vec{S}_2 \cdot \vec{v}_2 - 8 \vec{v}_2 \cdot \vec{v}_2 \hat{n} \times \vec{S}_1 \cdot \vec{v}_2 \hat{n} \times \vec{S}_2 \cdot \vec{v}_1 + \right.$$

$$32 \vec{v}_2 \cdot \vec{v}_2 \hat{n} \times \vec{S}_1 \cdot \vec{v}_1 \hat{n} \times \vec{S}_2 \cdot \vec{v}_2 + 4 \vec{S}_1 \cdot \vec{S}_2 \vec{v}_1 \cdot \vec{v}_2 (\hat{n} \cdot \vec{v}_2)^2 + 2 \vec{S}_1 \cdot \vec{S}_2 \vec{v}_2 \cdot \vec{v}_2 (\hat{n} \cdot \vec{v}_2)^2 -$$

$$4 \vec{v}_1 \cdot \vec{v}_2 \hat{n} \cdot \vec{S}_1 \hat{n} \cdot \vec{v}_2 \vec{S}_2 \cdot \vec{v}_2 - 2 \vec{v}_2 \cdot \vec{v}_2 \hat{n} \cdot \vec{S}_1 \hat{n} \cdot \vec{v}_2 \vec{S}_2 \cdot \vec{v}_1 - 2 \vec{v}_2 \cdot \vec{v}_2 \hat{n} \cdot \vec{S}_1 \hat{n} \cdot \vec{v}_2 \vec{S}_2 \cdot \vec{v}_2 +$$

$$2 \vec{v}_2 \cdot \vec{v}_2 \hat{n} \cdot \vec{S}_1 \hat{n} \cdot \vec{v}_1 \vec{S}_2 \cdot \vec{v}_2 + 12 \vec{v}_1 \cdot \vec{v}_2 \vec{v}_2 \cdot \vec{v}_2 \hat{n} \cdot \vec{S}_1 \hat{n} \cdot \vec{S}_2 - \vec{S}_1 \cdot \vec{S}_2 (\vec{v}_2 \cdot \vec{v}_2)^2 +$$

$$\left. 8 \vec{v}_2 \cdot \vec{v}_2 \vec{S}_1 \cdot \vec{v}_2 \vec{S}_2 \cdot \vec{v}_1 - 3 \vec{v}_2 \cdot \vec{v}_2 \vec{S}_1 \cdot \vec{v}_1 \vec{S}_2 \cdot \vec{v}_2 + \vec{v}_2 \cdot \vec{v}_2 \vec{S}_1 \cdot \vec{v}_2 \vec{S}_2 \cdot \vec{v}_2 - 9 \vec{S}_1 \cdot \vec{S}_2 \vec{v}_1 \cdot \vec{v}_2 \vec{v}_2 \cdot \vec{v}_2 \right) \Bigg\}$$

{DiagS1S2[2, 1, 2],

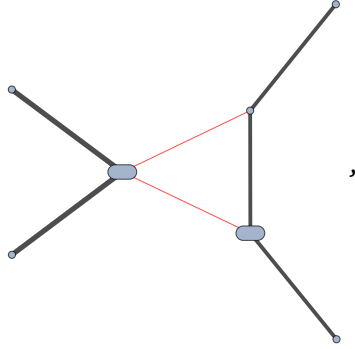

$$G^2 m_2 \left\{ \frac{-32 \vec{v}_1 \cdot \vec{v}_1 \hat{n} \times \vec{S}_1 \cdot \vec{v}_1 \hat{n} \times \vec{S}_2 \cdot \vec{v}_2 - 8 \vec{v}_1 \cdot \vec{v}_1 \vec{S}_1 \cdot \vec{v}_2 \vec{S}_2 \cdot \vec{v}_1 + 8 \vec{S}_1 \cdot \vec{S}_2 \vec{v}_1 \cdot \vec{v}_2 \vec{v}_1 \cdot \vec{v}_1}{r^4} - \frac{16 \vec{S}_1 \times \vec{v}_1 \cdot \vec{a}_1 \hat{n} \times \vec{S}_2 \cdot \vec{v}_2}{r^3} \right\}$$

{DiagS1S2[2, 1, 3],

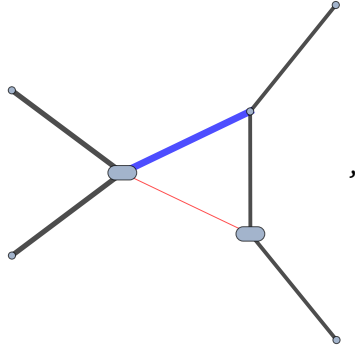

$$G^2 m_2 \left\{ \frac{24 \hat{n} \cdot \vec{v}_2 \vec{S}_1 \times \vec{v}_1 \cdot \vec{v}_2 \hat{n} \times \vec{S}_2 \cdot \vec{v}_2 - 24 \vec{v}_1 \cdot \vec{v}_2 \hat{n} \times \vec{S}_1 \cdot \vec{v}_2 \hat{n} \times \vec{S}_2 \cdot \vec{v}_2 - 8 \vec{v}_1 \cdot \vec{v}_2 \vec{S}_1 \cdot \vec{v}_2 \vec{S}_2 \cdot \vec{v}_2 + 8 \vec{S}_1 \cdot \vec{S}_2 \vec{v}_1 \cdot \vec{v}_2 \vec{v}_2 \cdot \vec{v}_2}{r^4} \right\}$$

{DiagS1S2[2, 1, 4],

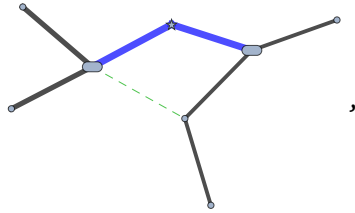

$$G^2 \left\{ \frac{1}{r^2} \left( \vec{S}_1 \cdot \vec{S}_2 (\hat{n} \cdot \vec{a}_2)^2 + \hat{n} \cdot \vec{v}_2 \vec{S}_1 \cdot \vec{S}_2 \hat{n} \cdot \vec{a}_2 + \hat{n} \cdot \vec{v}_2 \vec{S}_1 \cdot \vec{S}_2 \hat{n} \cdot \vec{a}_2 - \hat{n} \cdot \vec{S}_1 \vec{S}_2 \cdot \vec{a}_2 \hat{n} \cdot \vec{a}_2 - \right. \right.$$

$$\hat{n} \cdot \vec{S}_1 \vec{S}_2 \cdot \vec{v}_2 \hat{n} \cdot \vec{a}_2 + 3 \hat{n} \times \vec{S}_1 \cdot \vec{v}_2 \hat{n} \times \vec{S}_2 \cdot \vec{v}_2 + 4 \hat{n} \times \vec{S}_2 \cdot \vec{v}_2 \hat{n} \times \vec{S}_1 \cdot \vec{a}_2 - \hat{n} \times \vec{S}_2 \cdot \vec{a}_2 \hat{n} \times \vec{S}_1 \cdot \vec{v}_2 +$$

$$\left. 4 \hat{n} \times \vec{S}_1 \cdot \vec{v}_2 \hat{n} \times \vec{S}_2 \cdot \vec{a}_2 + 3 \hat{n} \times \vec{S}_1 \cdot \vec{a}_2 \hat{n} \times \vec{S}_2 \cdot \vec{a}_2 - \hat{n} \times \vec{S}_1 \cdot \vec{a}_2 \hat{n} \times \vec{S}_2 \cdot \vec{v}_2 + (\hat{n} \cdot \vec{v}_2)^2 \vec{S}_1 \cdot \vec{S}_2 - \right.$$

$gS1S2[2, 1, 5],$

$$\begin{aligned} G^2 & \left( \frac{1}{r^2} \left( 3 \hat{n} \times \vec{S}_2 \cdot \vec{v}_2 \hat{n} \times \vec{S}_1 \cdot \vec{a}_2 + 3 \hat{n} \times \vec{S}_2 \cdot \vec{a}_2 \hat{n} \times \vec{S}_1 \cdot \vec{v}_2 + 3 \hat{n} \times \vec{S}_1 \cdot \vec{v}_2 \hat{n} \times \vec{S}_2 \cdot \vec{a}_2 + 3 \hat{n} \times \vec{S}_1 \cdot \vec{a}_2 \hat{n} \times \vec{S}_2 \cdot \vec{v}_2 + \right. \right. \\ & 6 \hat{n} \cdot \vec{a}_2 \hat{n} \cdot \vec{v}_2 \vec{S}_1 \cdot \vec{S}_2 - 3 \hat{n} \cdot \vec{S}_1 \hat{n} \cdot \vec{v}_2 \vec{S}_2 \cdot \vec{a}_2 - 3 \hat{n} \cdot \vec{a}_2 \hat{n} \cdot \vec{S}_1 \vec{S}_2 \cdot \vec{v}_2 + 6 \hat{n} \cdot \vec{a}_2 \hat{n} \cdot \vec{v}_2 \vec{S}_1 \cdot \vec{S}_2 + \\ & 2 \vec{S}_2 \cdot \vec{v}_2 \vec{S}_1 \cdot \vec{a}_2 + 2 \vec{S}_2 \cdot \vec{a}_2 \vec{S}_1 \cdot \vec{v}_2 - 3 \hat{n} \cdot \vec{S}_1 \hat{n} \cdot \vec{v}_2 \vec{S}_2 \cdot \vec{a}_2 + 2 \vec{S}_1 \cdot \vec{v}_2 \vec{S}_2 \cdot \vec{a}_2 - 3 \hat{n} \cdot \vec{S}_1 \hat{n} \cdot \vec{a}_2 \vec{S}_2 \cdot \vec{v}_2 + \\ & \left. 2 \vec{S}_1 \cdot \vec{a}_2 \vec{S}_2 \cdot \vec{v}_2 + 12 \hat{n} \cdot \vec{S}_2 \hat{n} \cdot \vec{S}_1 \vec{v}_2 \cdot \vec{a}_2 + 12 \hat{n} \cdot \vec{S}_1 \hat{n} \cdot \vec{S}_2 \vec{v}_2 \cdot \vec{a}_2 - 8 \vec{S}_1 \cdot \vec{S}_2 \vec{v}_2 \cdot \vec{a}_2 - 8 \vec{S}_1 \cdot \vec{S}_2 \vec{v}_2 \cdot \vec{a}_2 \right) + \\ & \frac{1}{r^3} \left( -3 \vec{S}_1 \cdot \vec{S}_2 (\hat{n} \cdot \vec{v}_2)^3 - 3 \vec{S}_1 \cdot \vec{S}_2 (\hat{n} \cdot \vec{v}_2)^3 + 3 \hat{n} \cdot \vec{S}_1 \vec{S}_2 \cdot \vec{v}_2 (\hat{n} \cdot \vec{v}_2)^2 + 30 \hat{n} \cdot \vec{a}_2 \vec{S}_1 \cdot \vec{S}_2 (\hat{n} \cdot \vec{v}_2)^2 - \right. \\ & 15 \hat{n} \cdot \vec{S}_1 \vec{S}_2 \cdot \vec{a}_2 (\hat{n} \cdot \vec{v}_2)^2 + 3 \hat{n} \cdot \vec{S}_1 \vec{S}_2 \cdot \vec{v}_2 (\hat{n} \cdot \vec{v}_2)^2 - 3 \hat{n} \times \vec{S}_2 \cdot \vec{v}_2 \hat{n} \times \vec{S}_1 \cdot \vec{v}_2 \hat{n} \cdot \vec{v}_2 + \\ & \left. 15 \hat{n} \times \vec{S}_1 \cdot \vec{v}_2 \hat{n} \times \vec{S}_2 \cdot \vec{a}_2 \hat{n} \cdot \vec{v}_2 - 3 \hat{n} \times \vec{S}_1 \cdot \vec{v}_2 \hat{n} \times \vec{S}_2 \cdot \vec{v}_2 \hat{n} \cdot \vec{v}_2 + 15 \hat{n} \times \vec{S}_1 \cdot \vec{a}_2 \hat{n} \times \vec{S}_2 \cdot \vec{v}_2 \hat{n} \cdot \vec{v}_2 - \right. \end{aligned}$$





$$\begin{aligned} & 6 \vec{S}_1 \cdot \vec{S}_2 \vec{v}_1 \cdot \vec{v}_2 \hat{n} \cdot \vec{v}_2 + 14 \vec{S}_1 \cdot \vec{S}_2 \vec{v}_2 \cdot \vec{a}_2 \hat{n} \cdot \vec{v}_2 - 2 \vec{S}_1 \cdot \vec{S}_2 \vec{v}_2 \cdot \vec{v}_2 \hat{n} \cdot \vec{v}_2 - 2 \hat{n} \times \vec{S}_2 \cdot \vec{v}_1 \vec{S}_1 \times \vec{v}_1 \cdot \vec{a}_2 - \\ & 2 \hat{n} \times \vec{S}_1 \cdot \vec{a}_2 \vec{S}_2 \times \vec{v}_1 \cdot \vec{v}_2 - 8 \hat{n} \times \vec{S}_1 \cdot \vec{a}_2 \hat{n} \times \vec{S}_2 \cdot \vec{v}_1 \hat{n} \cdot \vec{v}_1 + 4 \hat{n} \cdot \vec{v}_1 \vec{S}_1 \cdot \vec{v}_2 \vec{S}_2 \cdot \vec{a}_2 - 8 \hat{n} \cdot \vec{a}_2 \hat{n} \cdot \vec{S}_1 \hat{n} \cdot \vec{v}_1 \vec{S}_2 \cdot \vec{v}_2 + \\ & 2 \hat{n} \cdot \vec{a}_2 \vec{S}_1 \cdot \vec{v}_1 \vec{S}_2 \cdot \vec{v}_2 - 2 \hat{n} \cdot \vec{a}_2 \vec{S}_1 \cdot \vec{v}_2 \vec{S}_2 \cdot \vec{v}_2 - 24 \hat{n} \cdot \vec{S}_1 \hat{n} \cdot \vec{S}_2 \hat{n} \cdot \vec{v}_1 \vec{v}_1 \cdot \vec{a}_2 + 4 \hat{n} \cdot \vec{v}_1 \vec{S}_1 \cdot \vec{S}_2 \vec{v}_1 \cdot \vec{a}_2 + \\ & 6 \hat{n} \cdot \vec{S}_2 \vec{S}_1 \cdot \vec{v}_1 \vec{v}_1 \cdot \vec{a}_2 - 6 \hat{n} \cdot \vec{S}_2 \vec{S}_1 \cdot \vec{v}_2 \vec{v}_1 \cdot \vec{a}_2 + 6 \hat{n} \cdot \vec{S}_1 \vec{S}_2 \cdot \vec{v}_1 \vec{v}_1 \cdot \vec{a}_2 - 4 \hat{n} \cdot \vec{S}_1 \vec{S}_2 \cdot \vec{v}_2 \vec{v}_1 \cdot \vec{a}_2 - \\ & 2 \hat{n} \cdot \vec{S}_1 \vec{S}_2 \cdot \vec{v}_2 \vec{v}_1 \cdot \vec{v}_2 - 12 \hat{n} \cdot \vec{a}_2 \vec{S}_1 \cdot \vec{S}_2 \vec{v}_1 \cdot \vec{v}_2 + 10 \hat{n} \cdot \vec{S}_1 \vec{S}_2 \cdot \vec{a}_2 \vec{v}_1 \cdot \vec{v}_2 - 4 \hat{n} \cdot \vec{v}_1 \vec{S}_1 \cdot \vec{S}_2 \vec{v}_2 \cdot \vec{a}_2 - \\ & 2 \hat{n} \cdot \vec{S}_1 \vec{S}_2 \cdot \vec{v}_2 \vec{v}_2 \cdot \vec{v}_2 + 8 \hat{n} \cdot \vec{a}_2 \vec{S}_1 \cdot \vec{S}_2 \vec{v}_2 \cdot \vec{v}_2 - 6 \hat{n} \cdot \vec{S}_1 \vec{S}_2 \cdot \vec{a}_2 \vec{v}_2 \cdot \vec{v}_2 - 2 \hat{n} \cdot \vec{S}_1 \vec{S}_2 \cdot \vec{v}_2 \vec{v}_2 \cdot \vec{v}_2 \Big) + \frac{1}{r^4} \\ & \left( 24 \vec{S}_1 \cdot \vec{S}_2 (\hat{n} \cdot \vec{v}_2)^4 - 24 \hat{n} \cdot \vec{v}_1 \vec{S}_1 \cdot \vec{S}_2 (\hat{n} \cdot \vec{v}_2)^3 - 24 \hat{n} \cdot \vec{S}_1 \vec{S}_2 \cdot \vec{v}_2 (\hat{n} \cdot \vec{v}_2)^3 + 6 \hat{n} \times \vec{S}_1 \cdot \vec{v}_2 \hat{n} \times \vec{S}_2 \cdot \vec{v}_1 (\hat{n} \cdot \vec{v}_2)^2 + \right. \\ & 24 \hat{n} \cdot \vec{S}_1 \hat{n} \cdot \vec{v}_1 \vec{S}_2 \cdot \vec{v}_2 (\hat{n} \cdot \vec{v}_2)^2 - 4 \vec{S}_1 \cdot \vec{v}_1 \vec{S}_2 \cdot \vec{v}_2 (\hat{n} \cdot \vec{v}_2)^2 + 10 \vec{S}_1 \cdot \vec{v}_2 \vec{S}_2 \cdot \vec{v}_2 (\hat{n} \cdot \vec{v}_2)^2 - 30 \hat{n} \cdot \vec{S}_1 \hat{n} \cdot \vec{S}_2 \\ & \vec{v}_1 \cdot \vec{v}_2 (\hat{n} \cdot \vec{v}_2)^2 + 18 \vec{S}_1 \cdot \vec{S}_2 \vec{v}_1 \cdot \vec{v}_2 (\hat{n} \cdot \vec{v}_2)^2 - 10 \vec{S}_1 \cdot \vec{S}_2 \vec{v}_2 \cdot \vec{v}_2 (\hat{n} \cdot \vec{v}_2)^2 - 2 \hat{n} \times \vec{S}_2 \cdot \vec{v}_1 \vec{S}_1 \times \vec{v}_1 \cdot \vec{v}_2 \hat{n} \cdot \vec{v}_2 - \\ & 2 \hat{n} \times \vec{S}_1 \cdot \vec{v}_2 \vec{S}_2 \times \vec{v}_1 \cdot \vec{v}_2 \hat{n} \cdot \vec{v}_2 - 12 \hat{n} \times \vec{S}_1 \cdot \vec{v}_2 \hat{n} \times \vec{S}_2 \cdot \vec{v}_1 \hat{n} \cdot \vec{v}_1 \hat{n} \cdot \vec{v}_2 - 8 \hat{n} \cdot \vec{v}_1 \vec{S}_1 \cdot \vec{v}_2 \vec{S}_2 \cdot \vec{v}_2 \hat{n} \cdot \vec{v}_2 + \\ & 36 \hat{n} \cdot \vec{S}_1 \hat{n} \cdot \vec{S}_2 \hat{n} \cdot \vec{v}_1 \vec{v}_1 \cdot \vec{v}_2 \hat{n} \cdot \vec{v}_2 - 8 \hat{n} \cdot \vec{v}_1 \vec{S}_1 \cdot \vec{S}_2 \vec{v}_1 \cdot \vec{v}_2 \hat{n} \cdot \vec{v}_2 - 6 \hat{n} \cdot \vec{S}_2 \vec{S}_1 \cdot \vec{v}_1 \vec{v}_1 \cdot \vec{v}_2 \hat{n} \cdot \vec{v}_2 + \\ & 6 \hat{n} \cdot \vec{S}_2 \vec{S}_1 \cdot \vec{v}_2 \vec{v}_1 \cdot \vec{v}_2 \hat{n} \cdot \vec{v}_2 - 6 \hat{n} \cdot \vec{S}_1 \vec{S}_2 \cdot \vec{v}_1 \vec{v}_1 \cdot \vec{v}_2 \hat{n} \cdot \vec{v}_2 - 2 \hat{n} \cdot \vec{S}_1 \vec{S}_2 \cdot \vec{v}_2 \vec{v}_1 \cdot \vec{v}_2 \hat{n} \cdot \vec{v}_2 - \\ & 6 \hat{n} \cdot \vec{S}_1 \hat{n} \cdot \vec{S}_2 (\vec{v}_1 \cdot \vec{v}_2)^2 + 2 \vec{S}_1 \cdot \vec{S}_2 (\vec{v}_1 \cdot \vec{v}_2)^2 - 2 \vec{S}_1 \cdot \vec{S}_2 (\vec{v}_2 \cdot \vec{v}_2)^2 + 2 \hat{n} \times \vec{S}_1 \cdot \vec{v}_2 \hat{n} \times \vec{S}_2 \cdot \vec{v}_1 \vec{v}_1 \cdot \vec{v}_2 + \\ & \left. 2 \vec{S}_1 \cdot \vec{v}_2 \vec{S}_2 \cdot \vec{v}_2 \vec{v}_1 \cdot \vec{v}_2 + 8 \hat{n} \cdot \vec{S}_1 \hat{n} \cdot \vec{v}_1 \vec{S}_2 \cdot \vec{v}_2 \vec{v}_2 \cdot \vec{v}_2 - 2 \vec{S}_1 \cdot \vec{v}_1 \vec{S}_2 \cdot \vec{v}_2 \vec{v}_2 \cdot \vec{v}_2 + 2 \vec{S}_1 \cdot \vec{v}_2 \vec{S}_2 \cdot \vec{v}_2 \vec{v}_2 \cdot \vec{v}_2 \right) \Big) m_2 \} \end{aligned}$$

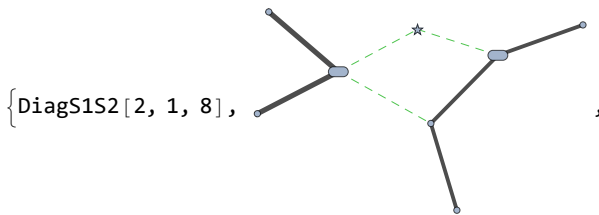

[illegible]

$\{\text{DiagS1S2}[2, 1, 9],$

$$\begin{aligned}
G^2 & \left( \frac{1}{r^2} \left( \vec{S}_1 \cdot \vec{S}_2 (\hat{n} \cdot \vec{a}_2)^2 + \hat{n} \cdot \vec{v}_2 \vec{S}_1 \cdot \vec{S}_2 \hat{n} \cdot \vec{a}_2 + \hat{n} \cdot \vec{v}_2 \vec{S}_1 \cdot \vec{S}_2 \hat{n} \cdot \vec{a}_2 - \hat{n} \cdot \vec{S}_1 \vec{S}_2 \cdot \vec{a}_2 \hat{n} \cdot \vec{a}_2 + \right. \right. \\
& 4 \hat{n} \times \vec{S}_2 \cdot \vec{v}_2 \hat{n} \times \vec{S}_1 \cdot \vec{a}_2 - \hat{n} \times \vec{S}_2 \cdot \vec{a}_2 \hat{n} \times \vec{S}_1 \cdot \vec{v}_2 - \hat{n} \times \vec{S}_1 \cdot \vec{v}_2 \hat{n} \times \vec{S}_2 \cdot \vec{a}_2 + 3 \hat{n} \times \vec{S}_1 \cdot \vec{a}_2 \hat{n} \times \vec{S}_2 \cdot \vec{a}_2 + \\
& 4 \hat{n} \times \vec{S}_1 \cdot \vec{a}_2 \hat{n} \times \vec{S}_2 \cdot \vec{v}_2 - \hat{n} \cdot \vec{S}_1 \hat{n} \cdot \vec{v}_2 \vec{S}_2 \cdot \vec{a}_2 + \hat{n} \cdot \vec{S}_1 \hat{n} \cdot \vec{S}_2 \vec{a}_2 \cdot \vec{a}_2 - \vec{a}_2 \cdot \vec{a}_2 \vec{S}_1 \cdot \vec{S}_2 - \\
& \left. \hat{n} \cdot \vec{S}_1 \hat{n} \cdot \vec{v}_2 \vec{S}_2 \cdot \vec{a}_2 + \hat{n} \cdot \vec{S}_2 \hat{n} \cdot \vec{S}_1 \vec{v}_2 \cdot \vec{a}_2 + \hat{n} \cdot \vec{S}_1 \hat{n} \cdot \vec{S}_2 \vec{v}_2 \cdot \vec{a}_2 - \vec{S}_1 \cdot \vec{S}_2 \vec{v}_2 \cdot \vec{a}_2 - \vec{S}_1 \cdot \vec{S}_2 \vec{v}_2 \cdot \vec{a}_2 \right) + \frac{1}{r^3} \\
& \left( \frac{1}{\vec{S}_1 \cdot \vec{S}_2} (\hat{n} \cdot \vec{v}_2)^3 + \vec{S}_1 \cdot \vec{S}_2 (\hat{n} \cdot \vec{v}_2)^3 - \hat{n} \cdot \vec{S}_1 \vec{S}_2 \cdot \vec{v}_2 (\hat{n} \cdot \vec{v}_2)^2 + 4 \hat{n} \cdot \vec{a}_2 \vec{S}_1 \cdot \vec{S}_2 (\hat{n} \cdot \vec{v}_2)^2 - 3 \hat{n} \cdot \vec{S}_1 \vec{S}_2 \cdot \vec{a}_2 (\hat{n} \cdot \vec{v}_2)^2 - \right. \\
& \hat{n} \cdot \vec{S}_1 \vec{S}_2 \cdot \vec{v}_2 (\hat{n} \cdot \vec{v}_2)^2 + 3 \hat{n} \times \vec{S}_2 \cdot \vec{v}_2 \hat{n} \times \vec{S}_1 \cdot \vec{v}_2 \hat{n} \cdot \vec{v}_2 + \hat{n} \times \vec{S}_1 \cdot \vec{v}_2 \hat{n} \times \vec{S}_2 \cdot \vec{a}_2 \hat{n} \cdot \vec{v}_2 + 3 \hat{n} \times \vec{S}_1 \cdot \vec{v}_2 \hat{n} \times \vec{S}_2 \cdot \vec{v}_2 \hat{n} \cdot \vec{v}_2 + \\
& 11 \hat{n} \times \vec{S}_1 \cdot \vec{a}_2 \hat{n} \times \vec{S}_2 \cdot \vec{v}_2 \hat{n} \cdot \vec{v}_2 - 4 \hat{n} \cdot \vec{a}_2 \hat{n} \cdot \vec{v}_1 \vec{S}_1 \cdot \vec{S}_2 \hat{n} \cdot \vec{v}_2 + 4 \hat{n} \cdot \vec{S}_1 \hat{n} \cdot \vec{v}_1 \vec{S}_2 \cdot \vec{a}_2 \hat{n} \cdot \vec{v}_2 - \vec{S}_1 \cdot \vec{v}_1 \vec{S}_2 \cdot \vec{a}_2 \hat{n} \cdot \vec{v}_2 + \\
& \vec{S}_1 \cdot \vec{v}_2 \vec{S}_2 \cdot \vec{a}_2 \hat{n} \cdot \vec{v}_2 - \hat{n} \cdot \vec{a}_2 \hat{n} \cdot \vec{S}_1 \vec{S}_2 \cdot \vec{v}_2 \hat{n} \cdot \vec{v}_2 + \vec{S}_1 \cdot \vec{S}_2 \vec{v}_1 \cdot \vec{a}_2 \hat{n} \cdot \vec{v}_2 + 4 \hat{n} \cdot \vec{S}_1 \hat{n} \cdot \vec{S}_2 \vec{v}_2 \cdot \vec{a}_2 \hat{n} \cdot \vec{v}_2 - \\
& 4 \vec{S}_1 \cdot \vec{S}_2 \vec{v}_2 \cdot \vec{a}_2 \hat{n} \cdot \vec{v}_2 + \hat{n} \cdot \vec{S}_2 \hat{n} \cdot \vec{S}_1 \vec{v}_2 \cdot \vec{v}_2 \hat{n} \cdot \vec{v}_2 + \hat{n} \cdot \vec{S}_1 \hat{n} \cdot \vec{S}_2 \vec{v}_2 \cdot \vec{v}_2 \hat{n} \cdot \vec{v}_2 - \vec{S}_1 \cdot \vec{S}_2 \vec{v}_2 \cdot \vec{v}_2 \hat{n} \cdot \vec{v}_2 - \\
& \vec{S}_1 \cdot \vec{S}_2 \vec{v}_2 \cdot \vec{v}_2 \hat{n} \cdot \vec{v}_2 - 4 \hat{n} \times \vec{S}_2 \cdot \vec{v}_2 \vec{S}_1 \times \vec{v}_1 \cdot \vec{a}_2 + \hat{n} \times \vec{S}_2 \cdot \vec{a}_2 \vec{S}_1 \times \vec{v}_1 \cdot \vec{v}_2 + \hat{n} \times \vec{S}_2 \cdot \vec{v}_2 \vec{S}_1 \times \vec{v}_2 \cdot \vec{a}_2 + \\
& \hat{n} \times \vec{S}_1 \cdot \vec{v}_2 \vec{S}_2 \times \vec{v}_1 \cdot \vec{a}_2 - 4 \hat{n} \times \vec{S}_1 \cdot \vec{a}_2 \vec{S}_2 \times \vec{v}_1 \cdot \vec{v}_2 - \hat{n} \times \vec{S}_1 \cdot \vec{v}_2 \vec{S}_2 \times \vec{v}_2 \cdot \vec{a}_2 + 4 \hat{n} \times \vec{S}_1 \cdot \vec{v}_2 \hat{n} \times \vec{S}_2 \cdot \vec{a}_2 \hat{n} \cdot \vec{v}_1 - \\
& 16 \hat{n} \times \vec{S}_1 \cdot \vec{a}_2 \hat{n} \times \vec{S}_2 \cdot \vec{v}_2 \hat{n} \cdot \vec{v}_1 + \hat{n} \cdot \vec{a}_2 \vec{S}_1 \cdot \vec{S}_2 \vec{v}_1 \cdot \vec{v}_2 - \hat{n} \cdot \vec{S}_1 \vec{S}_2 \cdot \vec{a}_2 \vec{v}_1 \cdot \vec{v}_2 - 4 \hat{n} \cdot \vec{S}_1 \hat{n} \cdot \vec{S}_2 \hat{n} \cdot \vec{v}_1 \vec{v}_2 \cdot \vec{a}_2 + \\
& \left. 2 \hat{n} \cdot \vec{v}_1 \vec{S}_1 \cdot \vec{S}_2 \vec{v}_2 \cdot \vec{a}_2 + \hat{n} \cdot \vec{S}_2 \vec{S}_1 \cdot \vec{v}_1 \vec{v}_2 \cdot \vec{a}_2 - \hat{n} \cdot \vec{S}_2 \vec{S}_1 \cdot \vec{v}_2 \vec{v}_2 \cdot \vec{a}_2 + \hat{n} \cdot \vec{S}_1 \vec{S}_2 \cdot \vec{v}_1 \vec{v}_2 \cdot \vec{a}_2 \right) + \frac{1}{r^4} \\
& \left( 3 \vec{S}_1 \cdot \vec{S}_2 (\hat{n} \cdot \vec{v}_2)^4 - 6 \hat{n} \cdot \vec{v}_1 \vec{S}_1 \cdot \vec{S}_2 (\hat{n} \cdot \vec{v}_2)^3 - 3 \hat{n} \cdot \vec{S}_1 \vec{S}_2 \cdot \vec{v}_2 (\hat{n} \cdot \vec{v}_2)^3 + 9 \hat{n} \times \vec{S}_1 \cdot \vec{v}_2 \hat{n} \times \vec{S}_2 \cdot \vec{v}_2 (\hat{n} \cdot \vec{v}_2)^2 + \right. \\
& 6 \hat{n} \cdot \vec{S}_1 \hat{n} \cdot \vec{v}_1 \vec{S}_2 \cdot \vec{v}_2 (\hat{n} \cdot \vec{v}_2)^2 - \vec{S}_1 \cdot \vec{v}_1 \vec{S}_2 \cdot \vec{v}_2 (\hat{n} \cdot \vec{v}_2)^2 + \vec{S}_1 \cdot \vec{v}_2 \vec{S}_2 \cdot \vec{v}_2 (\hat{n} \cdot \vec{v}_2)^2 +
\end{aligned}$$

$$\left. \begin{aligned} & 3 \vec{S}_1 \cdot \vec{S}_2 \vec{v}_1 \cdot \vec{v}_2 (\hat{n} \cdot \vec{v}_2)^2 + 3 \hat{n} \cdot \vec{S}_1 \hat{n} \cdot \vec{S}_2 \vec{v}_2 \cdot \vec{v}_2 (\hat{n} \cdot \vec{v}_2)^2 - 3 \vec{S}_1 \cdot \vec{S}_2 \vec{v}_2 \cdot \vec{v}_2 (\hat{n} \cdot \vec{v}_2)^2 - \\ & 3 \hat{n} \times \vec{S}_2 \cdot \vec{v}_2 \vec{S}_1 \times \vec{v}_1 \cdot \vec{v}_2 \hat{n} \cdot \vec{v}_2 - 3 \hat{n} \times \vec{S}_1 \cdot \vec{v}_2 \vec{S}_2 \times \vec{v}_1 \cdot \vec{v}_2 \hat{n} \cdot \vec{v}_2 - 18 \hat{n} \times \vec{S}_1 \cdot \vec{v}_2 \hat{n} \times \vec{S}_2 \cdot \vec{v}_2 \hat{n} \cdot \vec{v}_1 \hat{n} \cdot \vec{v}_2 - \\ & 2 \hat{n} \cdot \vec{S}_1 \vec{S}_2 \cdot \vec{v}_2 \vec{v}_1 \cdot \vec{v}_2 \hat{n} \cdot \vec{v}_2 - 6 \hat{n} \cdot \vec{S}_1 \hat{n} \cdot \vec{S}_2 \hat{n} \cdot \vec{v}_1 \vec{v}_2 \cdot \vec{v}_2 \hat{n} \cdot \vec{v}_2 + 4 \hat{n} \cdot \vec{v}_1 \vec{S}_1 \cdot \vec{S}_2 \vec{v}_2 \cdot \vec{v}_2 \hat{n} \cdot \vec{v}_2 + \\ & \hat{n} \cdot \vec{S}_2 \vec{S}_1 \cdot \vec{v}_1 \vec{v}_2 \cdot \vec{v}_2 \hat{n} \cdot \vec{v}_2 - \hat{n} \cdot \vec{S}_2 \vec{S}_1 \cdot \vec{v}_2 \vec{v}_2 \cdot \vec{v}_2 \hat{n} \cdot \vec{v}_2 + \hat{n} \cdot \vec{S}_1 \vec{S}_2 \cdot \vec{v}_1 \vec{v}_2 \cdot \vec{v}_2 \hat{n} \cdot \vec{v}_2 + \\ & 3 \hat{n} \times \vec{S}_1 \cdot \vec{v}_2 \hat{n} \times \vec{S}_2 \cdot \vec{v}_2 \vec{v}_1 \cdot \vec{v}_2 + \hat{n} \cdot \vec{S}_1 \hat{n} \cdot \vec{S}_2 \vec{v}_1 \cdot \vec{v}_2 \vec{v}_2 \cdot \vec{v}_2 - \vec{S}_1 \cdot \vec{S}_2 \vec{v}_1 \cdot \vec{v}_2 \vec{v}_2 \cdot \vec{v}_2 \end{aligned} \right) m_2 \}$$

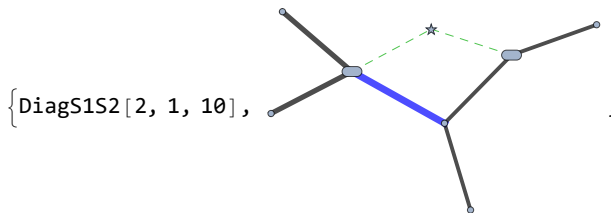

[illegible]

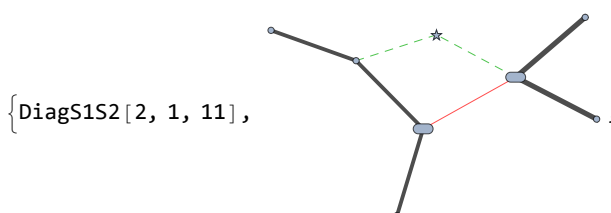

$$G^2 m_2 \left( \frac{1}{r^3} \left( 8 \vec{S}_1 \times \vec{v}_1 \cdot \vec{a}_2 \hat{n} \times \vec{S}_2 \cdot \vec{v}_2 + 8 \vec{S}_2 \times \vec{v}_1 \cdot \vec{v}_2 \hat{n} \times \vec{S}_1 \cdot \vec{a}_2 + 32 \hat{n} \cdot \vec{v}_1 \hat{n} \times \vec{S}_1 \cdot \vec{a}_2 \hat{n} \times \vec{S}_2 \cdot \vec{v}_2 - 8 \hat{n} \cdot \vec{v}_2 \hat{n} \times \vec{S}_2 \cdot \vec{a}_2 \hat{n} \times \vec{S}_1 \cdot \vec{v}_2 - \right. \right. \\ \left. \left. 24 \hat{n} \cdot \vec{v}_2 \hat{n} \times \vec{S}_1 \cdot \vec{a}_2 \hat{n} \times \vec{S}_2 \cdot \vec{v}_2 - 8 \hat{n} \cdot \vec{v}_2 \hat{n} \times \vec{S}_2 \cdot \vec{v}_2 \hat{n} \times \vec{S}_1 \cdot \vec{v}_2 - 8 \hat{n} \cdot \vec{v}_2 \hat{n} \times \vec{S}_1 \cdot \vec{v}_2 \hat{n} \times \vec{S}_2 \cdot \vec{v}_2 \right) + \right. \\ \left. \frac{-8 \hat{n} \times \vec{S}_1 \cdot \vec{a}_2 \hat{n} \times \vec{S}_2 \cdot \vec{v}_2 - 8 \hat{n} \times \vec{S}_1 \cdot \vec{a}_2 \hat{n} \times \vec{S}_2 \cdot \vec{v}_2 - 8 \hat{n} \times \vec{S}_2 \cdot \vec{a}_2 \hat{n} \times \vec{S}_1 \cdot \vec{a}_2}{r^2} + \frac{1}{r^4} \right. \\ \left. \left( -24 (\hat{n} \cdot \vec{v}_2)^2 \hat{n} \times \vec{S}_1 \cdot \vec{v}_2 \hat{n} \times \vec{S}_2 \cdot \vec{v}_2 + 8 \hat{n} \cdot \vec{v}_2 \vec{S}_1 \times \vec{v}_1 \cdot \vec{v}_2 \hat{n} \times \vec{S}_2 \cdot \vec{v}_2 + 8 \hat{n} \cdot \vec{v}_2 \vec{S}_2 \times \vec{v}_1 \cdot \vec{v}_2 \hat{n} \times \vec{S}_1 \cdot \vec{v}_2 + \right. \right. \\ \left. \left. 48 \hat{n} \cdot \vec{v}_1 \hat{n} \cdot \vec{v}_2 \hat{n} \times \vec{S}_1 \cdot \vec{v}_2 \hat{n} \times \vec{S}_2 \cdot \vec{v}_2 - 8 \vec{v}_1 \cdot \vec{v}_2 \hat{n} \times \vec{S}_1 \cdot \vec{v}_2 \hat{n} \times \vec{S}_2 \cdot \vec{v}_2 \right) \right) \Bigg\}$$

{DiagS1S2[2, 1, 12],

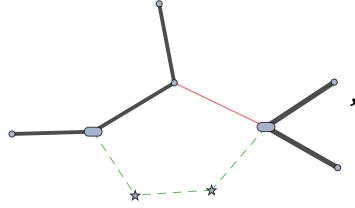

$$G^2 \left( \frac{1}{2} \hat{n} \cdot \vec{S}_1 \hat{n} \cdot \vec{S}_2 - \frac{3}{2} \vec{S}_1 \cdot \vec{S}_2 + \frac{1}{r} \left( - (\hat{n} \cdot \vec{S}_2) \hat{n} \cdot \vec{a}_1 \hat{n} \cdot \vec{S}_1 + \frac{1}{2} \hat{n} \cdot \vec{S}_2 \hat{n} \cdot \vec{a}_2 \hat{n} \cdot \vec{S}_1 + \right. \right. \\ \frac{1}{2} \vec{S}_2 \cdot \vec{a}_1 \hat{n} \cdot \vec{S}_1 + \frac{1}{2} \hat{n} \cdot \vec{S}_1 \hat{n} \cdot \vec{a}_2 \hat{n} \cdot \vec{S}_2 - 2 \hat{n} \cdot \vec{S}_1 \hat{n} \cdot \vec{S}_2 \hat{n} \cdot \vec{v}_1 + \hat{n} \cdot \vec{S}_1 \hat{n} \cdot \vec{S}_2 \hat{n} \cdot \vec{v}_2 + \hat{n} \cdot \vec{S}_1 \hat{n} \cdot \vec{S}_2 \hat{n} \cdot \vec{v}_2 - \\ 3 \hat{n} \cdot \vec{v}_2 \vec{S}_1 \cdot \vec{S}_2 + \hat{n} \cdot \vec{S}_2 \vec{S}_1 \cdot \vec{v}_1 + 3 \hat{n} \cdot \vec{v}_2 \vec{S}_1 \cdot \vec{S}_2 - \frac{1}{2} \hat{n} \cdot \vec{S}_2 \vec{S}_1 \cdot \vec{a}_2 + \frac{3}{2} \hat{n} \cdot \vec{a}_2 \vec{S}_1 \cdot \vec{S}_2 - \hat{n} \cdot \vec{S}_2 \vec{S}_1 \cdot \vec{v}_2 - \\ \hat{n} \cdot \vec{S}_1 \vec{S}_2 \cdot \vec{v}_2 + \hat{n} \cdot \vec{S}_1 \vec{S}_2 \cdot \vec{v}_1 - \frac{3}{2} \hat{n} \cdot \vec{a}_2 \vec{S}_1 \cdot \vec{S}_2 + \frac{1}{2} \hat{n} \cdot \vec{S}_2 \vec{S}_1 \cdot \vec{a}_1 - \frac{1}{2} \hat{n} \cdot \vec{S}_1 \vec{S}_2 \cdot \vec{a}_2 \Bigg) + \frac{1}{r^2} \\ \left( \frac{1}{2} \hat{n} \cdot \vec{S}_1 \hat{n} \cdot \vec{S}_2 (\hat{n} \cdot \vec{a}_2)^2 + \frac{3}{2} \vec{S}_1 \cdot \vec{S}_2 (\hat{n} \cdot \vec{a}_2)^2 - 2 \hat{n} \cdot \vec{a}_1 \hat{n} \cdot \vec{S}_1 \hat{n} \cdot \vec{S}_2 \hat{n} \cdot \vec{a}_2 - 4 \hat{n} \cdot \vec{S}_1 \hat{n} \cdot \vec{S}_2 \hat{n} \cdot \vec{v}_1 \hat{n} \cdot \vec{a}_2 + \right. \\ \hat{n} \cdot \vec{S}_2 \hat{n} \cdot \vec{S}_1 \hat{n} \cdot \vec{v}_2 \hat{n} \cdot \vec{a}_2 + \hat{n} \cdot \vec{S}_1 \hat{n} \cdot \vec{S}_2 \hat{n} \cdot \vec{v}_2 \hat{n} \cdot \vec{a}_2 - 6 \hat{n} \cdot \vec{v}_1 \vec{S}_1 \cdot \vec{S}_2 \hat{n} \cdot \vec{a}_2 + 3 \hat{n} \cdot \vec{v}_2 \vec{S}_1 \cdot \vec{S}_2 \hat{n} \cdot \vec{a}_2 + \\ \hat{n} \cdot \vec{S}_2 \vec{S}_1 \cdot \vec{v}_1 \hat{n} \cdot \vec{a}_2 - \hat{n} \cdot \vec{S}_1 \vec{S}_2 \cdot \vec{v}_2 \hat{n} \cdot \vec{a}_2 + 3 \hat{n} \cdot \vec{v}_2 \vec{S}_1 \cdot \vec{S}_2 \hat{n} \cdot \vec{a}_2 + \frac{1}{2} \hat{n} \cdot \vec{S}_2 \vec{S}_1 \cdot \vec{a}_1 \hat{n} \cdot \vec{a}_2 - \\ \frac{1}{2} \hat{n} \cdot \vec{S}_2 \vec{S}_1 \cdot \vec{a}_2 \hat{n} \cdot \vec{a}_2 - 3 \hat{n} \cdot \vec{a}_1 \vec{S}_1 \cdot \vec{S}_2 \hat{n} \cdot \vec{a}_2 - \hat{n} \cdot \vec{S}_2 \vec{S}_1 \cdot \vec{v}_2 \hat{n} \cdot \vec{a}_2 + \frac{1}{2} \hat{n} \cdot \vec{S}_1 \vec{S}_2 \cdot \vec{a}_1 \hat{n} \cdot \vec{a}_2 - \\ \frac{1}{2} \hat{n} \cdot \vec{S}_1 \vec{S}_2 \cdot \vec{a}_2 \hat{n} \cdot \vec{a}_2 + \hat{n} \cdot \vec{S}_1 \vec{S}_2 \cdot \vec{v}_1 \hat{n} \cdot \vec{a}_2 + 4 \hat{n} \cdot \vec{S}_2 \hat{n} \cdot \vec{S}_1 (\hat{n} \cdot \vec{v}_1)^2 + 2 \hat{n} \cdot \vec{S}_1 \hat{n} \cdot \vec{S}_2 (\hat{n} \cdot \vec{v}_2)^2 + \\ \frac{3}{2} \hat{n} \cdot \vec{S}_2 \hat{n} \cdot \vec{S}_1 (\hat{n} \cdot \vec{v}_2)^2 + \frac{3}{2} \hat{n} \cdot \vec{S}_1 \hat{n} \cdot \vec{S}_2 (\hat{n} \cdot \vec{v}_2)^2 - 4 \hat{n} \cdot \vec{S}_2 \hat{n} \cdot \vec{a}_1 \hat{n} \cdot \vec{S}_1 \hat{n} \cdot \vec{v}_2 - 8 \hat{n} \cdot \vec{S}_1 \hat{n} \cdot \vec{S}_2 \hat{n} \cdot \vec{v}_1 \hat{n} \cdot \vec{v}_2 - \\ 4 \hat{n} \cdot \vec{S}_2 \hat{n} \cdot \vec{S}_1 \hat{n} \cdot \vec{v}_1 \hat{n} \cdot \vec{v}_2 + 6 (\hat{n} \cdot \vec{v}_2)^2 \vec{S}_1 \cdot \vec{S}_2 - 12 \hat{n} \cdot \vec{v}_1 \hat{n} \cdot \vec{v}_2 \vec{S}_1 \cdot \vec{S}_2 + 2 \hat{n} \cdot \vec{S}_2 \hat{n} \cdot \vec{v}_1 \vec{S}_1 \cdot \vec{a}_2 - \\ \hat{n} \cdot \vec{S}_2 \hat{n} \cdot \vec{v}_2 \vec{S}_1 \cdot \vec{a}_2 + 2 \hat{n} \cdot \vec{S}_2 \hat{n} \cdot \vec{v}_2 \vec{S}_1 \cdot \vec{v}_1 + 4 \hat{n} \cdot \vec{S}_2 \hat{n} \cdot \vec{v}_1 \vec{S}_1 \cdot \vec{v}_2 - 2 \hat{n} \cdot \vec{S}_2 \hat{n} \cdot \vec{v}_2 \vec{S}_1 \cdot \vec{v}_2 + \frac{3}{2} (\hat{n} \cdot \vec{v}_2)^2 \vec{S}_1 \cdot \vec{S}_2 - \\ \hat{n} \cdot \vec{S}_2 \hat{n} \cdot \vec{v}_2 \vec{S}_1 \cdot \vec{v}_2 + \hat{n} \cdot \vec{S}_1 \hat{n} \cdot \vec{v}_2 \vec{S}_2 \cdot \vec{a}_1 + 2 \hat{n} \cdot \vec{S}_1 \hat{n} \cdot \vec{v}_2 \vec{S}_2 \cdot \vec{v}_1 - 2 \vec{S}_1 \cdot \vec{v}_2 \vec{S}_2 \cdot \vec{v}_1 + 2 \hat{n} \cdot \vec{a}_1 \hat{n} \cdot \vec{S}_1 \vec{S}_2 \cdot \vec{v}_2 + \\ 4 \hat{n} \cdot \vec{S}_1 \hat{n} \cdot \vec{v}_1 \vec{S}_2 \cdot \vec{v}_2 - 2 \hat{n} \cdot \vec{S}_1 \hat{n} \cdot \vec{v}_2 \vec{S}_2 \cdot \vec{v}_2 - 2 \vec{S}_1 \cdot \vec{v}_1 \vec{S}_2 \cdot \vec{v}_2 - 2 \hat{n} \cdot \vec{S}_1 \hat{n} \cdot \vec{v}_1 \vec{S}_2 \cdot \vec{v}_1 + \hat{n} \cdot \vec{S}_1 \hat{n} \cdot \vec{v}_2 \vec{S}_2 \cdot \vec{v}_1 + \\ \frac{1}{2} \hat{n} \cdot \vec{S}_1 \hat{n} \cdot \vec{S}_2 \vec{a}_1 \cdot \vec{a}_2 + \hat{n} \cdot \vec{S}_2 \hat{n} \cdot \vec{S}_1 \vec{a}_1 \cdot \vec{v}_2 - 6 \hat{n} \cdot \vec{a}_1 \hat{n} \cdot \vec{v}_2 \vec{S}_1 \cdot \vec{S}_2 + 3 \vec{a}_1 \cdot \vec{v}_2 \vec{S}_1 \cdot \vec{S}_2 - \frac{9}{2} (\hat{n} \cdot \vec{v}_2)^2 \vec{S}_1 \cdot \vec{S}_2 + \\ 6 \hat{n} \cdot \vec{v}_1 \hat{n} \cdot \vec{v}_2 \vec{S}_1 \cdot \vec{S}_2 + \hat{n} \cdot \vec{S}_2 \hat{n} \cdot \vec{v}_2 \vec{S}_1 \cdot \vec{a}_1 - \vec{S}_2 \cdot \vec{v}_2 \vec{S}_1 \cdot \vec{a}_1 + \hat{n} \cdot \vec{a}_1 \hat{n} \cdot \vec{S}_2 \vec{S}_1 \cdot \vec{a}_2 + \frac{3}{2} \vec{a}_1 \cdot \vec{a}_2 \vec{S}_1 \cdot \vec{S}_2 - \\ 2 \hat{n} \cdot \vec{S}_2 \hat{n} \cdot \vec{v}_1 \vec{S}_1 \cdot \vec{v}_1 + \hat{n} \cdot \vec{S}_2 \hat{n} \cdot \vec{v}_2 \vec{S}_1 \cdot \vec{v}_1 + \vec{S}_2 \cdot \vec{v}_1 \vec{S}_1 \cdot \vec{v}_1 + 2 \hat{n} \cdot \vec{S}_2 \hat{n} \cdot \vec{a}_1 \vec{S}_1 \cdot \vec{v}_2 - \vec{S}_2 \cdot \vec{a}_1 \vec{S}_1 \cdot \vec{v}_2 - \right.$$





$$\frac{1}{r^4}$$

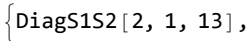

$G^2$

$$\frac{1}{r^4}$$

$$\begin{aligned} & \hat{n} \cdot \vec{S}_2 \vec{S}_1 \cdot \vec{v}_1 \vec{v}_1 \cdot \vec{v}_2 \hat{n} \cdot \vec{v}_2 - \hat{n} \cdot \vec{S}_2 \vec{S}_1 \cdot \vec{v}_2 \vec{v}_1 \cdot \vec{v}_2 \hat{n} \cdot \vec{v}_2 + 3 \hat{n} \cdot \vec{S}_1 \vec{S}_2 \cdot \vec{v}_1 \vec{v}_1 \cdot \vec{v}_2 \hat{n} \cdot \vec{v}_2 - 3 \hat{n} \cdot \vec{S}_1 \vec{S}_2 \cdot \vec{v}_2 \vec{v}_1 \cdot \vec{v}_2 \hat{n} \cdot \vec{v}_2 + \\ & 3 \hat{n} \cdot \vec{v}_1 \vec{S}_1 \cdot \vec{S}_2 \vec{v}_2 \cdot \vec{v}_2 \hat{n} \cdot \vec{v}_2 - 3 \hat{n} \cdot \vec{S}_1 \vec{S}_2 \cdot \vec{v}_1 \vec{v}_2 \cdot \vec{v}_2 \hat{n} \cdot \vec{v}_2 + \hat{n} \cdot \vec{S}_1 \hat{n} \cdot \vec{S}_2 \left( \vec{v}_1 \cdot \vec{v}_2 \right)^2 + \vec{S}_1 \times \vec{v}_1 \cdot \vec{v}_2 \vec{S}_2 \times \vec{v}_1 \cdot \vec{v}_2 + \\ & 4 \hat{n} \times \vec{S}_2 \cdot \vec{v}_2 \vec{S}_1 \times \vec{v}_1 \cdot \vec{v}_2 \hat{n} \cdot \vec{v}_1 - \hat{n} \times \vec{S}_1 \cdot \vec{v}_2 \hat{n} \times \vec{S}_2 \cdot \vec{v}_1 \vec{v}_1 \cdot \vec{v}_2 + 4 \hat{n} \cdot \vec{S}_1 \hat{n} \cdot \vec{v}_1 \vec{S}_2 \cdot \vec{v}_2 \vec{v}_1 \cdot \vec{v}_2 - \\ & \vec{S}_1 \cdot \vec{v}_1 \vec{S}_2 \cdot \vec{v}_2 \vec{v}_1 \cdot \vec{v}_2 + \vec{S}_1 \cdot \vec{v}_2 \vec{S}_2 \cdot \vec{v}_2 \vec{v}_1 \cdot \vec{v}_2 - 4 \left( \hat{n} \cdot \vec{v}_1 \right)^2 \vec{S}_1 \cdot \vec{S}_2 \vec{v}_2 \cdot \vec{v}_2 + 4 \hat{n} \cdot \vec{S}_1 \hat{n} \cdot \vec{v}_1 \vec{S}_2 \cdot \vec{v}_1 \vec{v}_2 \cdot \vec{v}_2 - \\ & \vec{S}_1 \cdot \vec{v}_1 \vec{S}_2 \cdot \vec{v}_1 \vec{v}_2 \cdot \vec{v}_2 + \vec{S}_1 \cdot \vec{v}_2 \vec{S}_2 \cdot \vec{v}_1 \vec{v}_2 \cdot \vec{v}_2 + \vec{S}_1 \cdot \vec{S}_2 \vec{v}_1 \cdot \vec{v}_1 \vec{v}_2 \cdot \vec{v}_2 - 2 \vec{S}_1 \cdot \vec{S}_2 \vec{v}_1 \cdot \vec{v}_2 \vec{v}_2 \cdot \vec{v}_2 \Big) \Big) m_2 \} \end{aligned}$$

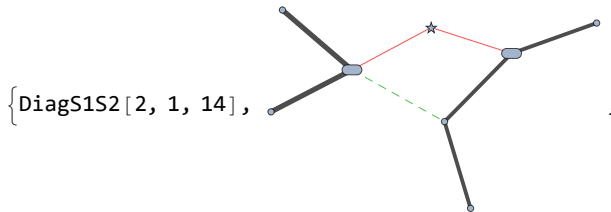

$$G^2 m_2 \left( \frac{1}{r^3} \left( 8 \vec{S}_1 \times \vec{v}_1 \cdot \vec{v}_2 \hat{n} \times \vec{S}_2 \cdot \vec{a}_2 + 8 \vec{S}_2 \times \vec{v}_1 \cdot \vec{a}_2 \hat{n} \times \vec{S}_1 \cdot \vec{v}_2 + 32 \hat{n} \cdot \vec{v}_1 \hat{n} \times \vec{S}_2 \cdot \vec{a}_2 \hat{n} \times \vec{S}_1 \cdot \vec{v}_2 - \right. \right. \\ \left. \left. 24 \hat{n} \cdot \vec{v}_2 \hat{n} \times \vec{S}_2 \cdot \vec{a}_2 \hat{n} \times \vec{S}_1 \cdot \vec{v}_2 - 8 \hat{n} \cdot \vec{v}_2 \hat{n} \times \vec{S}_1 \cdot \vec{a}_2 \hat{n} \times \vec{S}_2 \cdot \vec{v}_2 + 8 \vec{S}_2 \times \vec{v}_1 \cdot \vec{v}_2 \hat{n} \times \vec{S}_1 \cdot \vec{v}_2 + 8 \vec{S}_1 \times \vec{v}_1 \cdot \vec{v}_2 \hat{n} \times \vec{S}_2 \cdot \vec{v}_2 + \right. \right. \\ \left. \left. 32 \hat{n} \cdot \vec{v}_1 \hat{n} \times \vec{S}_2 \cdot \vec{v}_2 \hat{n} \times \vec{S}_1 \cdot \vec{v}_2 - 24 \hat{n} \cdot \vec{v}_2 \hat{n} \times \vec{S}_2 \cdot \vec{v}_2 \hat{n} \times \vec{S}_1 \cdot \vec{v}_2 - 8 \hat{n} \cdot \vec{v}_2 \hat{n} \times \vec{S}_1 \cdot \vec{v}_2 \hat{n} \times \vec{S}_2 \cdot \vec{v}_2 \right) + \right. \\ \left. \frac{-8 \hat{n} \times \vec{S}_1 \cdot \vec{a}_2 \hat{n} \times \vec{S}_2 \cdot \vec{v}_2 - 8 \hat{n} \times \vec{S}_2 \cdot \vec{a}_2 \hat{n} \times \vec{S}_1 \cdot \vec{v}_2 - 8 \hat{n} \times \vec{S}_1 \cdot \vec{a}_2 \hat{n} \times \vec{S}_2 \cdot \vec{a}_2 - 8 \hat{n} \times \vec{S}_1 \cdot \vec{v}_2 \hat{n} \times \vec{S}_2 \cdot \vec{v}_2}{r^2} + \right. \\ \left. \frac{1}{r^4} \left( -24 \left( \hat{n} \cdot \vec{v}_2 \right)^2 \hat{n} \times \vec{S}_1 \cdot \vec{v}_2 \hat{n} \times \vec{S}_2 \cdot \vec{v}_2 + 8 \hat{n} \cdot \vec{v}_2 \vec{S}_1 \times \vec{v}_1 \cdot \vec{v}_2 \hat{n} \times \vec{S}_2 \cdot \vec{v}_2 + \right. \right. \\ \left. \left. 8 \hat{n} \cdot \vec{v}_2 \vec{S}_2 \times \vec{v}_1 \cdot \vec{v}_2 \hat{n} \times \vec{S}_1 \cdot \vec{v}_2 + 48 \hat{n} \cdot \vec{v}_1 \hat{n} \cdot \vec{v}_2 \hat{n} \times \vec{S}_1 \cdot \vec{v}_2 \hat{n} \times \vec{S}_2 \cdot \vec{v}_2 - 8 \vec{v}_1 \cdot \vec{v}_2 \hat{n} \times \vec{S}_1 \cdot \vec{v}_2 \hat{n} \times \vec{S}_2 \cdot \vec{v}_2 \right) \right) \Bigg\}$$

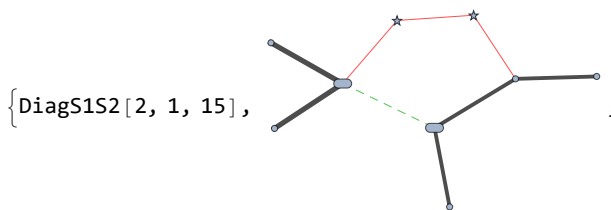

$$G^2 \left( \frac{-3 \hat{n} \cdot \vec{S_1} \hat{n} \cdot \vec{S_2} \hat{n} \cdot \vec{a_2} - \frac{3}{2} \hat{n} \cdot \vec{S_2} \hat{n} \cdot \vec{S_1} \hat{n} \cdot \vec{a_2} - \frac{3}{2} \hat{n} \cdot \vec{S_1} \hat{n} \cdot \vec{S_2} \hat{n} \cdot \vec{a_2} + \frac{1}{2} \vec{S_1} \cdot \vec{S_2} \hat{n} \cdot \vec{a_2} + \frac{1}{2} \vec{S_1} \cdot \vec{S_2} \hat{n} \cdot \vec{a_2}}{r} + \right.$$

$$\frac{1}{r^2} \left( -\frac{15}{2} \hat{n} \cdot \vec{S_1} \hat{n} \cdot \vec{S_2} (\hat{n} \cdot \vec{a_2})^2 + \frac{3}{2} \vec{S_1} \cdot \vec{S_2} (\hat{n} \cdot \vec{a_2})^2 + 6 \hat{n} \cdot \vec{a_1} \hat{n} \cdot \vec{S_1} \hat{n} \cdot \vec{S_2} \hat{n} \cdot \vec{a_2} + 12 \hat{n} \cdot \vec{S_2} \hat{n} \cdot \vec{S_1} \hat{n} \cdot \vec{v_1} \hat{n} \cdot \vec{a_2} + \right.$$

$$12 \hat{n} \cdot \vec{S_1} \hat{n} \cdot \vec{S_2} \hat{n} \cdot \vec{v_1} \hat{n} \cdot \vec{a_2} - 15 \hat{n} \cdot \vec{S_2} \hat{n} \cdot \vec{S_1} \hat{n} \cdot \vec{v_2} \hat{n} \cdot \vec{a_2} - 15 \hat{n} \cdot \vec{S_1} \hat{n} \cdot \vec{S_2} \hat{n} \cdot \vec{v_2} \hat{n} \cdot \vec{a_2} - 2 \hat{n} \cdot \vec{v_1} \vec{S_1} \cdot \vec{S_2} \hat{n} \cdot \vec{a_2} +$$

$$3 \hat{n} \cdot \vec{v_2} \vec{S_1} \cdot \vec{S_2} \hat{n} \cdot \vec{a_2} - 3 \hat{n} \cdot \vec{S_2} \vec{S_1} \cdot \vec{v_1} \hat{n} \cdot \vec{a_2} + 3 \hat{n} \cdot \vec{S_2} \vec{S_1} \cdot \vec{v_2} \hat{n} \cdot \vec{a_2} - 3 \hat{n} \cdot \vec{S_1} \vec{S_2} \cdot \vec{v_1} \hat{n} \cdot \vec{a_2} + 3 \hat{n} \cdot \vec{S_1} \vec{S_2} \cdot \vec{v_2} \hat{n} \cdot \vec{a_2} -$$

$$2 \hat{n} \cdot \vec{v_1} \vec{S_1} \cdot \vec{S_2} \hat{n} \cdot \vec{a_2} + 3 \hat{n} \cdot \vec{v_2} \vec{S_1} \cdot \vec{S_2} \hat{n} \cdot \vec{a_2} - \frac{3}{2} \hat{n} \cdot \vec{S_2} \vec{S_1} \cdot \vec{a_1} \hat{n} \cdot \vec{a_2} + \frac{3}{2} \hat{n} \cdot \vec{S_2} \vec{S_1} \cdot \vec{a_2} \hat{n} \cdot \vec{a_2} - \hat{n} \cdot \vec{a_1} \vec{S_1} \cdot \vec{S_2} \hat{n} \cdot \vec{a_2} -$$

$$3 \hat{n} \cdot \vec{S_2} \vec{S_1} \cdot \vec{v_1} \hat{n} \cdot \vec{a_2} + 3 \hat{n} \cdot \vec{S_2} \vec{S_1} \cdot \vec{v_2} \hat{n} \cdot \vec{a_2} - \frac{3}{2} \hat{n} \cdot \vec{S_1} \vec{S_2} \cdot \vec{a_1} \hat{n} \cdot \vec{a_2} + \frac{3}{2} \hat{n} \cdot \vec{S_1} \vec{S_2} \cdot \vec{a_2} \hat{n} \cdot \vec{a_2} - 3 \hat{n} \cdot \vec{S_1} \vec{S_2} \cdot \vec{v_1} \hat{n} \cdot \vec{a_2} +$$

$$3 \hat{n} \cdot \vec{S_1} \vec{S_2} \cdot \vec{v_2} \hat{n} \cdot \vec{a_2} + 3 \hat{n} \cdot \vec{S_1} \hat{n} \cdot \vec{S_2} (\hat{n} \cdot \vec{v_2})^2 + \frac{3}{2} \hat{n} \cdot \vec{S_2} \hat{n} \cdot \vec{S_1} (\hat{n} \cdot \vec{v_2})^2 + \frac{3}{2} \hat{n} \cdot \vec{S_1} \hat{n} \cdot \vec{S_2} (\hat{n} \cdot \vec{v_2})^2 -$$

$$(\hat{n} \cdot \vec{v_2})^2 \vec{S_1} \cdot \vec{S_2} - \frac{1}{2} (\hat{n} \cdot \vec{v_2})^2 \vec{S_1} \cdot \vec{S_2} - \frac{3}{2} \hat{n} \cdot \vec{S_1} \hat{n} \cdot \vec{S_2} \vec{a_1} \cdot \vec{a_2} - \frac{1}{2} (\hat{n} \cdot \vec{v_2})^2 \vec{S_1} \cdot \vec{S_2} + \frac{1}{2} \vec{a_1} \cdot \vec{a_2} \vec{S_1} \cdot \vec{S_2} -$$



$$\left. \begin{aligned} & 12 \hat{n} \cdot \vec{S}_2 \hat{n} \cdot \vec{v}_1 \vec{S}_1 \cdot \vec{v}_2 \vec{v}_2 \cdot \vec{v}_2 - 12 \hat{n} \cdot \vec{S}_1 \hat{n} \cdot \vec{v}_1 \vec{S}_2 \cdot \vec{v}_1 \vec{v}_2 \cdot \vec{v}_2 + 3 \vec{S}_1 \cdot \vec{v}_1 \vec{S}_2 \cdot \vec{v}_1 \vec{v}_2 \cdot \vec{v}_2 - \\ & 3 \vec{S}_1 \cdot \vec{v}_2 \vec{S}_2 \cdot \vec{v}_1 \vec{v}_2 \cdot \vec{v}_2 + 12 \hat{n} \cdot \vec{S}_1 \hat{n} \cdot \vec{v}_1 \vec{S}_2 \cdot \vec{v}_2 \vec{v}_2 \cdot \vec{v}_2 - 3 \vec{S}_1 \cdot \vec{v}_1 \vec{S}_2 \cdot \vec{v}_2 \vec{v}_2 \cdot \vec{v}_2 + 3 \vec{S}_1 \cdot \vec{v}_2 \vec{S}_2 \cdot \vec{v}_2 \vec{v}_2 \cdot \vec{v}_2 - \\ & 6 \hat{n} \cdot \vec{S}_1 \hat{n} \cdot \vec{S}_2 \vec{v}_1 \cdot \vec{v}_1 \vec{v}_2 \cdot \vec{v}_2 + \vec{S}_1 \cdot \vec{S}_2 \vec{v}_1 \cdot \vec{v}_1 \vec{v}_2 \cdot \vec{v}_2 + 15 \hat{n} \cdot \vec{S}_1 \hat{n} \cdot \vec{S}_2 \vec{v}_1 \cdot \vec{v}_2 \vec{v}_2 \cdot \vec{v}_2 - 3 \vec{S}_1 \cdot \vec{S}_2 \vec{v}_1 \cdot \vec{v}_2 \vec{v}_2 \cdot \vec{v}_2 \end{aligned} \right\} m_2 \}$$

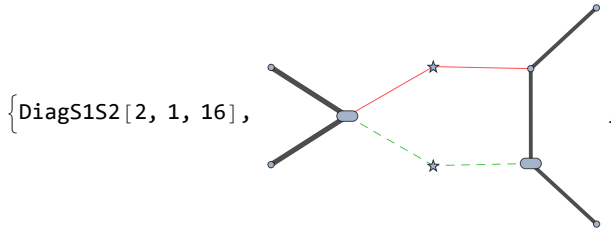

[illegible]

[illegible]

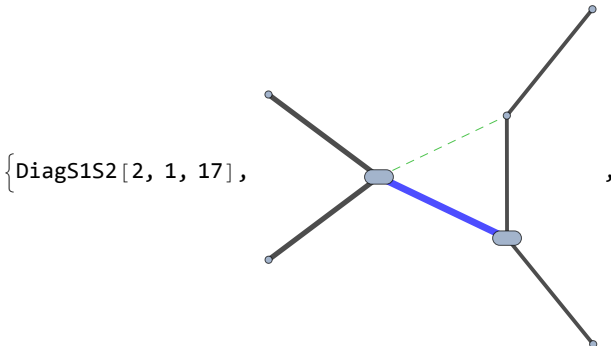



{DiagS1S2[2, 1, 19],

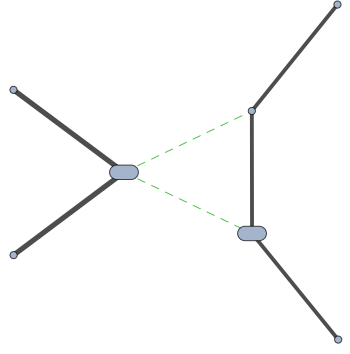

,

$$\begin{aligned}
 G^2 \left( \frac{1}{r^2} \left( 16 \vec{S}_2 \cdot \vec{v}_2 \vec{S}_1 \cdot \vec{a}_2 - 8 \vec{S}_2 \cdot \vec{a}_2 \vec{S}_1 \cdot \vec{a}_2 + 8 \vec{a}_2 \cdot \vec{a}_2 \vec{S}_1 \cdot \vec{S}_2 - 8 \vec{S}_2 \cdot \vec{a}_2 \vec{S}_1 \cdot \vec{v}_2 + \right. \right. \\
 \left. \left. 8 \vec{S}_2 \cdot \vec{v}_2 \vec{S}_1 \cdot \vec{v}_2 + 8 \vec{S}_1 \cdot \vec{a}_2 \vec{S}_2 \cdot \vec{v}_2 - 8 \vec{S}_1 \cdot \vec{S}_2 \vec{v}_2 \cdot \vec{a}_2 - 8 \vec{S}_1 \cdot \vec{S}_2 \vec{v}_2 \cdot \vec{a}_2 - 8 \vec{S}_1 \cdot \vec{S}_2 \vec{v}_2 \cdot \vec{v}_2 \right) + \frac{1}{r^3} \right. \\
 \left. \left( -8 \hat{n} \times \vec{S}_1 \cdot \vec{v}_2 \vec{S}_2 \times \vec{v}_1 \cdot \vec{v}_2 - 6 \hat{n} \times \vec{S}_2 \cdot \vec{v}_1 \vec{S}_1 \times \vec{v}_1 \cdot \vec{a}_2 + 6 \hat{n} \times \vec{S}_2 \cdot \vec{v}_1 \vec{S}_1 \times \vec{v}_1 \cdot \vec{v}_2 - 12 \hat{n} \times \vec{S}_2 \cdot \vec{v}_2 \vec{S}_1 \times \vec{v}_2 \cdot \vec{a}_2 - \right. \right. \\
 \left. \left. 8 \hat{n} \times \vec{S}_1 \cdot \vec{v}_2 \vec{S}_2 \times \vec{v}_1 \cdot \vec{a}_2 + 2 \hat{n} \cdot \vec{v}_2 \vec{S}_2 \cdot \vec{v}_2 \vec{S}_1 \cdot \vec{v}_2 - 2 \hat{n} \cdot \vec{v}_2 \vec{S}_1 \cdot \vec{v}_2 \vec{S}_2 \cdot \vec{a}_2 + \right. \right. \\
 \left. \left. 2 \hat{n} \cdot \vec{v}_2 \vec{S}_1 \cdot \vec{a}_2 \vec{S}_2 \cdot \vec{v}_2 + 2 \hat{n} \cdot \vec{a}_2 \vec{S}_1 \cdot \vec{v}_2 \vec{S}_2 \cdot \vec{v}_2 - 6 \hat{n} \cdot \vec{v}_1 \vec{S}_1 \cdot \vec{S}_2 \vec{v}_1 \cdot \vec{a}_2 + 6 \hat{n} \cdot \vec{S}_1 \vec{S}_2 \cdot \vec{v}_1 \vec{v}_1 \cdot \vec{a}_2 - \right. \right. \\
 \left. \left. 6 \hat{n} \cdot \vec{S}_1 \vec{S}_2 \cdot \vec{v}_1 \vec{v}_1 \cdot \vec{v}_2 + 6 \hat{n} \cdot \vec{v}_1 \vec{S}_1 \cdot \vec{S}_2 \vec{v}_1 \cdot \vec{v}_2 - 8 \hat{n} \cdot \vec{v}_2 \vec{S}_1 \cdot \vec{S}_2 \vec{v}_1 \cdot \vec{v}_2 + 8 \hat{n} \cdot \vec{S}_2 \vec{S}_1 \cdot \vec{a}_2 \vec{v}_1 \cdot \vec{v}_2 - \right. \right. \\
 \left. \left. 8 \hat{n} \cdot \vec{a}_2 \vec{S}_1 \cdot \vec{S}_2 \vec{v}_1 \cdot \vec{v}_2 + 8 \hat{n} \cdot \vec{S}_2 \vec{S}_1 \cdot \vec{v}_2 \vec{v}_1 \cdot \vec{v}_2 - 4 \hat{n} \cdot \vec{v}_2 \vec{S}_1 \cdot \vec{S}_2 \vec{v}_2 \cdot \vec{a}_2 + 4 \hat{n} \cdot \vec{S}_1 \vec{S}_2 \cdot \vec{v}_2 \vec{v}_2 \cdot \vec{a}_2 - \right. \right. \\
 \left. \left. 2 \hat{n} \cdot \vec{S}_1 \vec{S}_2 \cdot \vec{v}_2 \vec{v}_2 \cdot \vec{v}_2 - 4 \hat{n} \cdot \vec{a}_2 \vec{S}_1 \cdot \vec{S}_2 \vec{v}_2 \cdot \vec{v}_2 + 2 \hat{n} \cdot \vec{S}_1 \vec{S}_2 \cdot \vec{a}_2 \vec{v}_2 \cdot \vec{v}_2 \right) + \frac{1}{r^4} \right. \\
 \left. \left( -18 \vec{S}_1 \cdot \vec{S}_2 \vec{v}_1 \cdot \vec{v}_2 (\hat{n} \cdot \vec{v}_1)^2 + 6 \hat{n} \times \vec{S}_2 \cdot \vec{v}_1 \vec{S}_1 \times \vec{v}_1 \cdot \vec{v}_2 \hat{n} \cdot \vec{v}_1 + 12 \hat{n} \cdot \vec{v}_2 \vec{S}_1 \cdot \vec{S}_2 \vec{v}_1 \cdot \vec{v}_2 \hat{n} \cdot \vec{v}_1 + \right. \right. \\
 \left. \left. 18 \hat{n} \cdot \vec{S}_1 \vec{S}_2 \cdot \vec{v}_1 \vec{v}_1 \cdot \vec{v}_2 \hat{n} \cdot \vec{v}_1 - 6 \vec{S}_1 \cdot \vec{S}_2 (\vec{v}_1 \cdot \vec{v}_2)^2 - 6 \vec{S}_1 \times \vec{v}_1 \cdot \vec{v}_2 \vec{S}_2 \times \vec{v}_1 \cdot \vec{v}_2 + \right. \right. \\
 \left. \left. 12 \hat{n} \times \vec{S}_2 \cdot \vec{v}_1 \vec{S}_1 \times \vec{v}_1 \cdot \vec{v}_2 \hat{n} \cdot \vec{v}_2 - 2 \hat{n} \times \vec{S}_1 \cdot \vec{v}_2 \vec{S}_2 \times \vec{v}_1 \cdot \vec{v}_2 \hat{n} \cdot \vec{v}_2 + 4 (\hat{n} \cdot \vec{v}_2)^2 \vec{S}_1 \cdot \vec{v}_2 \vec{S}_2 \cdot \vec{v}_2 - \right. \right. \\
 \left. \left. 24 \hat{n} \times \vec{S}_1 \cdot \vec{v}_1 \hat{n} \times \vec{S}_2 \cdot \vec{v}_1 \vec{v}_1 \cdot \vec{v}_2 + 24 \hat{n} \times \vec{S}_1 \cdot \vec{v}_2 \hat{n} \times \vec{S}_2 \cdot \vec{v}_2 \vec{v}_1 \cdot \vec{v}_2 - 6 (\hat{n} \cdot \vec{v}_2)^2 \vec{S}_1 \cdot \vec{S}_2 \vec{v}_1 \cdot \vec{v}_2 + \right. \right. \\
 \left. \left. 6 \hat{n} \cdot \vec{S}_2 \hat{n} \cdot \vec{v}_2 \vec{S}_1 \cdot \vec{v}_2 \vec{v}_1 \cdot \vec{v}_2 - 12 \hat{n} \cdot \vec{S}_1 \hat{n} \cdot \vec{v}_2 \vec{S}_2 \cdot \vec{v}_1 \vec{v}_1 \cdot \vec{v}_2 - 12 \vec{S}_1 \cdot \vec{v}_1 \vec{S}_2 \cdot \vec{v}_1 \vec{v}_1 \cdot \vec{v}_2 + \right. \right. \\
 \left. \left. 6 \vec{S}_1 \cdot \vec{v}_2 \vec{S}_2 \cdot \vec{v}_1 \vec{v}_1 \cdot \vec{v}_2 + 4 \vec{S}_1 \cdot \vec{v}_2 \vec{S}_2 \cdot \vec{v}_2 \vec{v}_1 \cdot \vec{v}_2 + 12 \vec{S}_1 \cdot \vec{S}_2 \vec{v}_1 \cdot \vec{v}_1 \vec{v}_1 \cdot \vec{v}_2 + 2 \hat{n} \times \vec{S}_1 \cdot \vec{v}_2 \hat{n} \times \vec{S}_2 \cdot \vec{v}_1 \vec{v}_2 \cdot \vec{v}_2 - \right. \right. \\
 \left. \left. 4 \hat{n} \cdot \vec{S}_1 \hat{n} \cdot \vec{v}_2 \vec{S}_2 \cdot \vec{v}_2 \vec{v}_2 \cdot \vec{v}_2 - 6 \hat{n} \cdot \vec{S}_1 \hat{n} \cdot \vec{S}_2 \vec{v}_1 \cdot \vec{v}_2 \vec{v}_2 \cdot \vec{v}_2 - 2 \vec{S}_1 \cdot \vec{S}_2 \vec{v}_1 \cdot \vec{v}_2 \vec{v}_2 \cdot \vec{v}_2 \right) \right) m_2 \}
 \end{aligned}$$

{DiagS1S2[2, 1, 20],

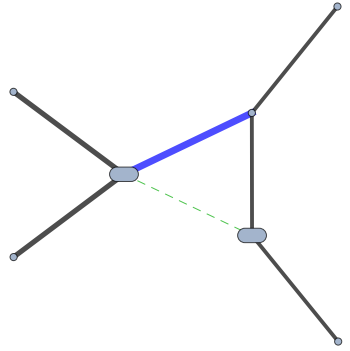

,

$$\begin{aligned}
 G^2 \left( \frac{1}{r^3} \left( -4 \hat{n} \times \vec{S}_2 \cdot \vec{v}_2 \vec{S}_1 \times \vec{v}_1 \cdot \vec{v}_2 + 4 \hat{n} \times \vec{S}_1 \cdot \vec{v}_2 \vec{S}_2 \times \vec{v}_2 \cdot \vec{a}_2 - 4 \hat{n} \cdot \vec{v}_2 \vec{S}_2 \cdot \vec{v}_2 \vec{S}_1 \cdot \vec{v}_2 - 4 \hat{n} \cdot \vec{v}_2 \vec{S}_1 \cdot \vec{a}_2 \vec{S}_2 \cdot \vec{v}_2 + \right. \right. \\
 \left. \left. 4 \hat{n} \cdot \vec{v}_2 \vec{S}_1 \cdot \vec{S}_2 \vec{v}_1 \cdot \vec{a}_2 - 4 \hat{n} \cdot \vec{S}_1 \vec{S}_2 \cdot \vec{v}_2 \vec{v}_1 \cdot \vec{a}_2 + 4 \hat{n} \cdot \vec{S}_1 \vec{S}_2 \cdot \vec{v}_2 \vec{v}_1 \cdot \vec{v}_2 - 4 \hat{n} \cdot \vec{v}_2 \vec{S}_1 \cdot \vec{S}_2 \vec{v}_1 \cdot \vec{v}_2 + 4 \hat{n} \cdot \vec{a}_2 \vec{S}_1 \cdot \vec{S}_2 \right. \right. \\
 \left. \left. \vec{v}_1 \cdot \vec{v}_2 - 4 \hat{n} \cdot \vec{S}_1 \vec{S}_2 \cdot \vec{a}_2 \vec{v}_1 \cdot \vec{v}_2 - 8 \hat{n} \cdot \vec{v}_1 \vec{S}_1 \cdot \vec{S}_2 \vec{v}_2 \cdot \vec{a}_2 + 4 \hat{n} \cdot \vec{v}_2 \vec{S}_1 \cdot \vec{S}_2 \vec{v}_2 \cdot \vec{a}_2 + 8 \hat{n} \cdot \vec{S}_1 \vec{S}_2 \cdot \vec{v}_1 \vec{v}_2 \cdot \vec{a}_2 - \right. \right. \\
 \left. \left. 4 \hat{n} \cdot \vec{v}_2 \vec{S}_1 \cdot \vec{S}_2 \vec{v}_2 \cdot \vec{v}_2 + 8 \hat{n} \cdot \vec{S}_2 \vec{S}_1 \cdot \vec{a}_2 \vec{v}_2 \cdot \vec{v}_2 - 8 \hat{n} \cdot \vec{a}_2 \vec{S}_1 \cdot \vec{S}_2 \vec{v}_2 \cdot \vec{v}_2 + 8 \hat{n} \cdot \vec{S}_2 \vec{S}_1 \cdot \vec{v}_2 \vec{v}_2 \cdot \vec{v}_2 \right) + \frac{1}{r^4} \right.
 \end{aligned}$$



$$\left( -3 \vec{S}_1 \cdot \vec{v}_2 \vec{S}_2 \cdot \vec{v}_2 (\hat{n} \cdot \vec{v}_2)^2 - 8 \vec{S}_1 \cdot \vec{S}_2 \vec{v}_1 \cdot \vec{v}_2 (\hat{n} \cdot \vec{v}_2)^2 - 6 \vec{S}_1 \cdot \vec{S}_2 \vec{v}_2 \cdot \vec{v}_2 (\hat{n} \cdot \vec{v}_2)^2 - 9 \hat{n} \times \vec{S}_2 \cdot \vec{v}_1 \vec{S}_1 \times \vec{v}_1 \cdot \vec{v}_2 \hat{n} \cdot \vec{v}_2 - \right. \\ \left. 12 \hat{n} \times \vec{S}_2 \cdot \vec{v}_2 \vec{S}_1 \times \vec{v}_1 \cdot \vec{v}_2 \hat{n} \cdot \vec{v}_2 + 9 \hat{n} \cdot \vec{v}_1 \vec{S}_1 \cdot \vec{S}_2 \vec{v}_1 \cdot \vec{v}_2 \hat{n} \cdot \vec{v}_2 + 8 \hat{n} \cdot \vec{S}_1 \vec{S}_2 \cdot \vec{v}_2 \vec{v}_1 \cdot \vec{v}_2 \hat{n} \cdot \vec{v}_2 - \right. \\ \left. 4 \hat{n} \cdot \vec{v}_1 \vec{S}_1 \cdot \vec{S}_2 \vec{v}_2 \cdot \vec{v}_2 \hat{n} \cdot \vec{v}_2 + 6 \hat{n} \cdot \vec{S}_2 \vec{S}_1 \cdot \vec{v}_2 \vec{v}_2 \cdot \vec{v}_2 \hat{n} \cdot \vec{v}_2 + 4 \hat{n} \cdot \vec{S}_1 \vec{S}_2 \cdot \vec{v}_1 \vec{v}_2 \cdot \vec{v}_2 \hat{n} \cdot \vec{v}_2 + \right. \\ \left. 3 \hat{n} \cdot \vec{S}_1 \vec{S}_2 \cdot \vec{v}_2 \vec{v}_2 \cdot \vec{v}_2 \hat{n} \cdot \vec{v}_2 - 6 \vec{S}_1 \cdot \vec{S}_2 (\vec{v}_1 \cdot \vec{v}_2)^2 - 6 \hat{n} \cdot \vec{S}_1 \hat{n} \cdot \vec{S}_2 (\vec{v}_2 \cdot \vec{v}_2)^2 + 2 \vec{S}_1 \cdot \vec{S}_2 (\vec{v}_2 \cdot \vec{v}_2)^2 + \right. \\ \left. 6 \vec{S}_1 \times \vec{v}_1 \cdot \vec{v}_2 \vec{S}_2 \times \vec{v}_1 \cdot \vec{v}_2 + 9 \hat{n} \times \vec{S}_2 \cdot \vec{v}_2 \vec{S}_1 \times \vec{v}_1 \cdot \vec{v}_2 \hat{n} \cdot \vec{v}_1 + 9 \hat{n} \times \vec{S}_1 \cdot \vec{v}_2 \hat{n} \times \vec{S}_2 \cdot \vec{v}_1 \vec{v}_1 \cdot \vec{v}_2 - 9 \hat{n} \cdot \vec{S}_1 \hat{n} \cdot \vec{v}_1 \vec{S}_2 \cdot \vec{v}_2 \vec{v}_1 \cdot \vec{v}_2 + \right. \\ \left. 6 \vec{S}_1 \cdot \vec{v}_1 \vec{S}_2 \cdot \vec{v}_2 \vec{v}_1 \cdot \vec{v}_2 - 4 \vec{S}_1 \cdot \vec{v}_2 \vec{S}_2 \cdot \vec{v}_2 \vec{v}_1 \cdot \vec{v}_2 + 6 \hat{n} \times \vec{S}_1 \cdot \vec{v}_2 \hat{n} \times \vec{S}_2 \cdot \vec{v}_2 \vec{v}_2 \cdot \vec{v}_2 + 4 \vec{S}_1 \cdot \vec{S}_2 \vec{v}_1 \cdot \vec{v}_2 \vec{v}_2 \cdot \vec{v}_2 \right) m_2 \Bigg\}$$

{DiagS1S2[2, 1, 21],

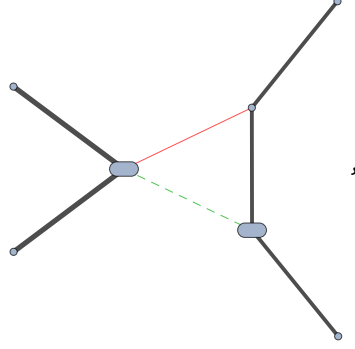

$$G^2 \left( \frac{1}{r^3} \left( 8 \hat{n} \times \vec{S}_2 \cdot \vec{v}_1 \vec{S}_1 \times \vec{v}_1 \cdot \vec{a}_1 + 8 \hat{n} \times \vec{S}_1 \cdot \vec{v}_2 \vec{S}_2 \times \vec{v}_2 \cdot \vec{a}_2 + 8 \hat{n} \cdot \vec{v}_2 \vec{S}_2 \cdot \vec{v}_1 \vec{S}_1 \cdot \vec{v}_2 + 8 \hat{n} \cdot \vec{v}_2 \vec{S}_1 \cdot \vec{a}_2 \vec{S}_2 \cdot \vec{v}_1 - \right. \right. \\ \left. \left. 8 \hat{n} \cdot \vec{v}_2 \vec{S}_1 \cdot \vec{S}_2 \vec{v}_1 \cdot \vec{a}_2 + 4 \hat{n} \cdot \vec{S}_1 \vec{S}_2 \cdot \vec{v}_1 \vec{v}_1 \cdot \vec{v}_1 - 4 \hat{n} \cdot \vec{v}_1 \vec{S}_1 \cdot \vec{S}_2 \vec{v}_1 \cdot \vec{v}_1 - 8 \hat{n} \cdot \vec{v}_2 \vec{S}_1 \cdot \vec{S}_2 \vec{v}_1 \cdot \vec{v}_2 + \right. \right. \\ \left. \left. 12 \hat{n} \cdot \vec{v}_1 \vec{S}_1 \cdot \vec{S}_2 \vec{v}_2 \cdot \vec{a}_2 + 8 \hat{n} \cdot \vec{v}_2 \vec{S}_1 \cdot \vec{S}_2 \vec{v}_2 \cdot \vec{a}_2 - 8 \hat{n} \cdot \vec{S}_2 \vec{S}_1 \cdot \vec{v}_2 \vec{v}_2 \cdot \vec{a}_2 - 12 \hat{n} \cdot \vec{S}_1 \vec{S}_2 \cdot \vec{v}_1 \vec{v}_2 \cdot \vec{a}_2 + \right. \right. \\ \left. \left. 16 \hat{n} \cdot \vec{v}_2 \vec{S}_1 \cdot \vec{S}_2 \vec{v}_2 \cdot \vec{v}_2 - 16 \hat{n} \cdot \vec{S}_2 \vec{S}_1 \cdot \vec{a}_2 \vec{v}_2 \cdot \vec{v}_2 + 16 \hat{n} \cdot \vec{a}_2 \vec{S}_1 \cdot \vec{S}_2 \vec{v}_2 \cdot \vec{v}_2 - 16 \hat{n} \cdot \vec{S}_2 \vec{S}_1 \cdot \vec{v}_2 \vec{v}_2 \cdot \vec{v}_2 \right) + \right. \\ \left. \frac{1}{r^4} \left( \frac{21}{2} \vec{S}_1 \cdot \vec{S}_2 \vec{v}_1 \cdot \vec{v}_1 (\hat{n} \cdot \vec{v}_1)^2 - 10 \hat{n} \cdot \vec{v}_2 \vec{S}_1 \cdot \vec{S}_2 \vec{v}_1 \cdot \vec{v}_1 \hat{n} \cdot \vec{v}_1 - \frac{21}{2} \hat{n} \cdot \vec{S}_1 \vec{S}_2 \cdot \vec{v}_1 \vec{v}_1 \cdot \vec{v}_1 \hat{n} \cdot \vec{v}_1 + \right. \right. \\ \left. \left. 6 \hat{n} \cdot \vec{v}_2 \vec{S}_1 \cdot \vec{S}_2 \vec{v}_2 \cdot \vec{v}_2 \hat{n} \cdot \vec{v}_1 - 7 \vec{S}_1 \cdot \vec{S}_2 (\vec{v}_1 \cdot \vec{v}_1)^2 + \frac{21}{2} \hat{n} \cdot \vec{S}_1 \hat{n} \cdot \vec{S}_2 (\vec{v}_2 \cdot \vec{v}_2)^2 + \frac{11}{2} \vec{S}_1 \cdot \vec{S}_2 (\vec{v}_2 \cdot \vec{v}_2)^2 - \right. \right. \\ \left. \left. 6 \hat{n} \times \vec{S}_2 \cdot \vec{v}_2 \vec{S}_1 \times \vec{v}_1 \cdot \vec{v}_2 \hat{n} \cdot \vec{v}_2 + 2 (\hat{n} \cdot \vec{v}_2)^2 \vec{S}_1 \cdot \vec{v}_2 \vec{S}_2 \cdot \vec{v}_1 + \frac{29}{2} \hat{n} \times \vec{S}_1 \cdot \vec{v}_1 \hat{n} \times \vec{S}_2 \cdot \vec{v}_1 \vec{v}_1 \cdot \vec{v}_1 + \right. \right. \\ \left. \left. 10 \hat{n} \cdot \vec{S}_1 \hat{n} \cdot \vec{v}_2 \vec{S}_2 \cdot \vec{v}_1 \vec{v}_1 \cdot \vec{v}_1 + 7 \vec{S}_1 \cdot \vec{v}_1 \vec{S}_2 \cdot \vec{v}_1 \vec{v}_1 \cdot \vec{v}_1 - 4 \vec{S}_1 \cdot \vec{v}_2 \vec{S}_2 \cdot \vec{v}_1 \vec{v}_1 \cdot \vec{v}_1 - 2 (\hat{n} \cdot \vec{v}_2)^2 \vec{S}_1 \cdot \vec{S}_2 \vec{v}_1 \cdot \vec{v}_2 + \right. \right. \\ \left. \left. 4 \vec{S}_1 \cdot \vec{S}_2 \vec{v}_1 \cdot \vec{v}_1 \vec{v}_1 \cdot \vec{v}_2 - \frac{75}{2} \hat{n} \times \vec{S}_1 \cdot \vec{v}_2 \hat{n} \times \vec{S}_2 \cdot \vec{v}_2 \vec{v}_2 \cdot \vec{v}_2 + \frac{21}{2} (\hat{n} \cdot \vec{v}_2)^2 \vec{S}_1 \cdot \vec{S}_2 \vec{v}_2 \cdot \vec{v}_2 - \right. \right. \\ \left. \left. \frac{21}{2} \hat{n} \cdot \vec{S}_2 \hat{n} \cdot \vec{v}_2 \vec{S}_1 \cdot \vec{v}_2 \vec{v}_2 \cdot \vec{v}_2 - 6 \hat{n} \cdot \vec{S}_1 \hat{n} \cdot \vec{v}_2 \vec{S}_2 \cdot \vec{v}_1 \vec{v}_2 \cdot \vec{v}_2 - 9 \vec{S}_1 \cdot \vec{v}_2 \vec{S}_2 \cdot \vec{v}_2 \vec{v}_2 \cdot \vec{v}_2 \right) \right) m_2 \Bigg\}$$

{DiagS1S2[2, 1, 22],

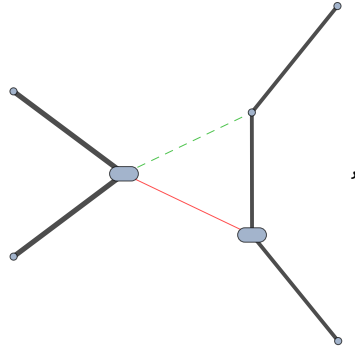

$$G^2 m_2 \left( \frac{-16 \vec{S}_1 \times \vec{v}_1 \cdot \vec{v}_2 \hat{n} \times \vec{S}_2 \cdot \vec{a}_2 + 16 \vec{S}_2 \times \vec{v}_2 \cdot \vec{a}_2 \hat{n} \times \vec{S}_1 \cdot \vec{v}_2 - 16 \vec{S}_1 \times \vec{v}_1 \cdot \vec{v}_2 \hat{n} \times \vec{S}_2 \cdot \vec{v}_2}{r^3} + \right.$$

$$\left. \frac{-48 \hat{n} \cdot \vec{v}_2 \vec{S}_1 \times \vec{v}_1 \cdot \vec{v}_2 \hat{n} \times \vec{S}_2 \cdot \vec{v}_2 - 16 \vec{v}_2 \cdot \vec{v}_2 \hat{n} \times \vec{S}_1 \cdot \vec{v}_2 \hat{n} \times \vec{S}_2 \cdot \vec{v}_2}{r^4} \right\}$$

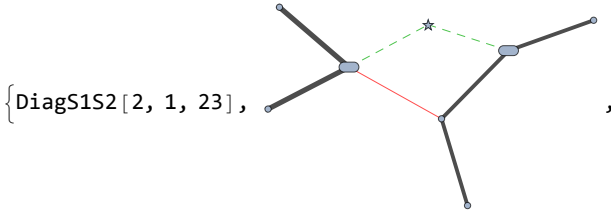

$$\left. \begin{aligned} & 6 \hat{n} \cdot \vec{S}_2 \vec{S}_1 \cdot \vec{v}_2 \vec{v}_2 \cdot \vec{a}_2 - 6 \hat{n} \cdot \vec{S}_1 \vec{S}_2 \cdot \vec{v}_2 \vec{v}_2 \cdot \vec{a}_2 - 12 \hat{n} \cdot \vec{S}_2 \hat{n} \cdot \vec{S}_1 \hat{n} \cdot \vec{v}_1 \vec{v}_2 \cdot \vec{v}_2 - 2 \hat{n} \cdot \vec{S}_2 \vec{S}_1 \cdot \vec{v}_2 \vec{v}_2 \cdot \vec{v}_2 + \\ & 5 \hat{n} \cdot \vec{S}_1 \vec{S}_2 \cdot \vec{v}_1 \vec{v}_2 \cdot \vec{v}_2 - 4 \hat{n} \cdot \vec{v}_1 \vec{S}_1 \cdot \vec{S}_2 \vec{v}_2 \cdot \vec{v}_2 + 3 \hat{n} \cdot \vec{S}_2 \vec{S}_1 \cdot \vec{v}_1 \vec{v}_2 \cdot \vec{v}_2 - 3 \hat{n} \cdot \vec{S}_1 \vec{S}_2 \cdot \vec{v}_2 \vec{v}_2 \cdot \vec{v}_2 \Big) + \frac{1}{r^4} \\ & \left( 3 \vec{S}_1 \cdot \vec{S}_2 (\hat{n} \cdot \vec{v}_2)^4 - 12 \hat{n} \cdot \vec{v}_1 \vec{S}_1 \cdot \vec{S}_2 (\hat{n} \cdot \vec{v}_2)^3 - 3 \hat{n} \cdot \vec{S}_2 \vec{S}_1 \cdot \vec{v}_2 (\hat{n} \cdot \vec{v}_2)^3 - 6 \hat{n} \cdot \vec{S}_1 \vec{S}_2 \cdot \vec{v}_1 (\hat{n} \cdot \vec{v}_2)^3 - \right. \\ & 9 \hat{n} \times \vec{S}_1 \cdot \vec{v}_2 \hat{n} \times \vec{S}_2 \cdot \vec{v}_2 (\hat{n} \cdot \vec{v}_2)^2 - 12 (\hat{n} \cdot \vec{v}_1)^2 \vec{S}_1 \cdot \vec{S}_2 (\hat{n} \cdot \vec{v}_2)^2 + 18 \hat{n} \cdot \vec{S}_2 \hat{n} \cdot \vec{v}_1 \vec{S}_1 \cdot \vec{v}_2 (\hat{n} \cdot \vec{v}_2)^2 + \\ & 12 \hat{n} \cdot \vec{S}_1 \hat{n} \cdot \vec{v}_1 \vec{S}_2 \cdot \vec{v}_1 (\hat{n} \cdot \vec{v}_2)^2 - 2 \vec{S}_1 \cdot \vec{v}_1 \vec{S}_2 \cdot \vec{v}_1 (\hat{n} \cdot \vec{v}_2)^2 + 3 \vec{S}_1 \cdot \vec{v}_2 \vec{S}_2 \cdot \vec{v}_1 (\hat{n} \cdot \vec{v}_2)^2 - \vec{S}_1 \cdot \vec{v}_2 \vec{S}_2 \cdot \vec{v}_2 (\hat{n} \cdot \vec{v}_2)^2 + \\ & 2 \vec{S}_1 \cdot \vec{S}_2 \vec{v}_1 \cdot \vec{v}_1 (\hat{n} \cdot \vec{v}_2)^2 + 3 \vec{S}_1 \cdot \vec{S}_2 \vec{v}_1 \cdot \vec{v}_2 (\hat{n} \cdot \vec{v}_2)^2 + 9 \hat{n} \cdot \vec{S}_1 \hat{n} \cdot \vec{S}_2 \vec{v}_2 \cdot \vec{v}_2 (\hat{n} \cdot \vec{v}_2)^2 + 3 \vec{S}_1 \cdot \vec{S}_2 \vec{v}_2 \cdot \vec{v}_2 (\hat{n} \cdot \vec{v}_2)^2 + \\ & 9 \hat{n} \times \vec{S}_2 \cdot \vec{v}_2 \vec{S}_1 \times \vec{v}_1 \cdot \vec{v}_2 \hat{n} \cdot \vec{v}_2 + 9 \hat{n} \times \vec{S}_1 \cdot \vec{v}_2 \vec{S}_2 \times \vec{v}_1 \cdot \vec{v}_2 \hat{n} \cdot \vec{v}_2 + 54 \hat{n} \times \vec{S}_1 \cdot \vec{v}_2 \hat{n} \times \vec{S}_2 \cdot \vec{v}_2 \hat{n} \cdot \vec{v}_1 \hat{n} \cdot \vec{v}_2 - \\ & 8 \hat{n} \cdot \vec{v}_1 \vec{S}_1 \cdot \vec{v}_2 \vec{S}_2 \cdot \vec{v}_1 \hat{n} \cdot \vec{v}_2 + 4 \hat{n} \cdot \vec{v}_1 \vec{S}_1 \cdot \vec{v}_2 \vec{S}_2 \cdot \vec{v}_2 \hat{n} \cdot \vec{v}_2 + 12 \hat{n} \cdot \vec{v}_1 \vec{S}_1 \cdot \vec{S}_2 \vec{v}_1 \cdot \vec{v}_2 \hat{n} \cdot \vec{v}_2 - \\ & 6 \hat{n} \cdot \vec{S}_2 \vec{S}_1 \cdot \vec{v}_2 \vec{v}_1 \cdot \vec{v}_2 \hat{n} \cdot \vec{v}_2 - 4 \hat{n} \cdot \vec{S}_1 \vec{S}_2 \cdot \vec{v}_1 \vec{v}_1 \cdot \vec{v}_2 \hat{n} \cdot \vec{v}_2 - 54 \hat{n} \cdot \vec{S}_1 \hat{n} \cdot \vec{S}_2 \hat{n} \cdot \vec{v}_1 \vec{v}_2 \cdot \vec{v}_2 \hat{n} \cdot \vec{v}_2 - \\ & 14 \hat{n} \cdot \vec{v}_1 \vec{S}_1 \cdot \vec{S}_2 \vec{v}_2 \cdot \vec{v}_2 \hat{n} \cdot \vec{v}_2 + 9 \hat{n} \cdot \vec{S}_2 \vec{S}_1 \cdot \vec{v}_1 \vec{v}_2 \cdot \vec{v}_2 \hat{n} \cdot \vec{v}_2 - 2 \hat{n} \cdot \vec{S}_2 \vec{S}_1 \cdot \vec{v}_2 \vec{v}_2 \cdot \vec{v}_2 \hat{n} \cdot \vec{v}_2 + \\ & 11 \hat{n} \cdot \vec{S}_1 \vec{S}_2 \cdot \vec{v}_1 \vec{v}_2 \cdot \vec{v}_2 \hat{n} \cdot \vec{v}_2 - 3 \hat{n} \cdot \vec{S}_1 \vec{S}_2 \cdot \vec{v}_2 \vec{v}_2 \cdot \vec{v}_2 \hat{n} \cdot \vec{v}_2 - 2 \vec{S}_1 \cdot \vec{S}_2 (\vec{v}_1 \cdot \vec{v}_2)^2 - 9 \hat{n} \times \vec{S}_1 \cdot \vec{v}_2 \hat{n} \times \vec{S}_2 \cdot \vec{v}_2 \vec{v}_1 \cdot \vec{v}_2 + \\ & 2 \vec{S}_1 \cdot \vec{v}_2 \vec{S}_2 \cdot \vec{v}_1 \vec{v}_1 \cdot \vec{v}_2 - \vec{S}_1 \cdot \vec{v}_2 \vec{S}_2 \cdot \vec{v}_2 \vec{v}_1 \cdot \vec{v}_2 + 8 \hat{n} \cdot \vec{S}_2 \hat{n} \cdot \vec{v}_1 \vec{S}_1 \cdot \vec{v}_2 \vec{v}_2 \cdot \vec{v}_2 - 4 \vec{S}_1 \cdot \vec{v}_2 \vec{S}_2 \cdot \vec{v}_1 \vec{v}_2 \cdot \vec{v}_2 + \\ & \left. 12 \hat{n} \cdot \vec{S}_1 \hat{n} \cdot \vec{v}_1 \vec{S}_2 \cdot \vec{v}_2 \vec{v}_2 \cdot \vec{v}_2 - 3 \vec{S}_1 \cdot \vec{v}_1 \vec{S}_2 \cdot \vec{v}_2 \vec{v}_2 \cdot \vec{v}_2 + 9 \hat{n} \cdot \vec{S}_1 \hat{n} \cdot \vec{S}_2 \vec{v}_1 \cdot \vec{v}_2 \vec{v}_2 \cdot \vec{v}_2 + 5 \vec{S}_1 \cdot \vec{S}_2 \vec{v}_1 \cdot \vec{v}_2 \vec{v}_2 \cdot \vec{v}_2 \right) \Bigg\} m_2 \end{aligned} \right)$$

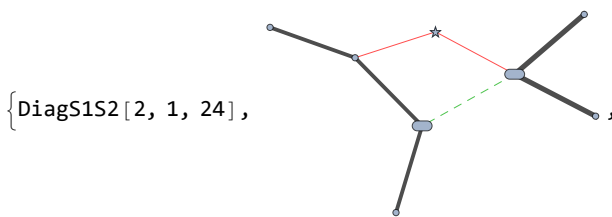

[illegible]



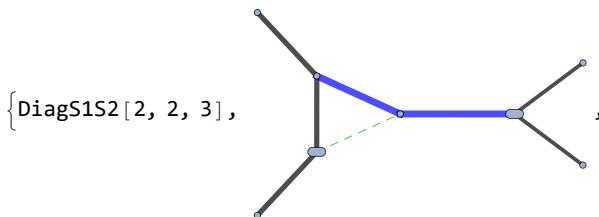

$$\begin{aligned} G^2 \left( \frac{1}{r^3} \right) & \left( -8 \hat{n} \times \vec{S}_1 \cdot \vec{v}_1 \vec{S}_2 \times \vec{v}_1 \cdot \vec{v}_2 - 8 \hat{n} \times \vec{S}_2 \cdot \vec{v}_1 \vec{S}_1 \times \vec{a}_1 \cdot \vec{v}_2 - 4 \hat{n} \times \vec{S}_2 \cdot \vec{v}_1 \vec{S}_1 \times \vec{v}_1 \cdot \vec{a}_2 - 4 \hat{n} \times \vec{S}_2 \cdot \vec{v}_1 \vec{S}_1 \times \vec{v}_1 \cdot \vec{v}_2 - \right. \\ & 8 \hat{n} \times \vec{S}_2 \cdot \vec{a}_1 \vec{S}_1 \times \vec{v}_1 \cdot \vec{v}_2 - 5 \hat{n} \times \vec{S}_1 \cdot \vec{v}_1 \vec{S}_2 \times \vec{a}_1 \cdot \vec{v}_2 - 8 \hat{n} \times \vec{S}_1 \cdot \vec{v}_1 \vec{S}_2 \times \vec{v}_1 \cdot \vec{a}_2 - 9 \hat{n} \times \vec{S}_1 \cdot \vec{v}_1 \vec{S}_2 \times \vec{v}_1 \cdot \vec{v}_2 - \\ & 5 \hat{n} \times \vec{S}_1 \cdot \vec{a}_1 \vec{S}_2 \times \vec{v}_1 \cdot \vec{v}_2 - 4 \hat{n} \times \vec{S}_1 \cdot \vec{v}_2 \hat{n} \times \vec{S}_2 \cdot \vec{v}_1 \hat{n} \cdot \vec{a}_1 + 8 \hat{n} \times \vec{S}_1 \cdot \vec{v}_1 \hat{n} \times \vec{S}_2 \cdot \vec{v}_2 \hat{n} \cdot \vec{a}_1 + 16 \hat{n} \times \vec{S}_1 \cdot \vec{v}_1 \hat{n} \times \vec{S}_2 \cdot \vec{v}_1 \hat{n} \cdot \vec{a}_2 - \\ & 16 \hat{n} \times \vec{S}_2 \cdot \vec{v}_2 \hat{n} \times \vec{S}_1 \cdot \vec{v}_1 \hat{n} \cdot \vec{v}_1 + 8 \hat{n} \times \vec{S}_2 \cdot \vec{v}_1 \hat{n} \times \vec{S}_1 \cdot \vec{v}_2 \hat{n} \cdot \vec{v}_1 - 4 \hat{n} \times \vec{S}_1 \cdot \vec{v}_2 \hat{n} \times \vec{S}_2 \cdot \vec{a}_1 \hat{n} \cdot \vec{v}_1 - \\ & 16 \hat{n} \times \vec{S}_1 \cdot \vec{v}_1 \hat{n} \times \vec{S}_2 \cdot \vec{a}_2 \hat{n} \cdot \vec{v}_1 + 12 \hat{n} \times \vec{S}_1 \cdot \vec{v}_2 \hat{n} \times \vec{S}_2 \cdot \vec{v}_1 \hat{n} \cdot \vec{v}_1 + 8 \hat{n} \times \vec{S}_1 \cdot \vec{a}_2 \hat{n} \times \vec{S}_2 \cdot \vec{v}_1 \hat{n} \cdot \vec{v}_1 - \\ & 24 \hat{n} \times \vec{S}_1 \cdot \vec{v}_1 \hat{n} \times \vec{S}_2 \cdot \vec{v}_2 \hat{n} \cdot \vec{v}_1 + 8 \hat{n} \times \vec{S}_1 \cdot \vec{a}_1 \hat{n} \times \vec{S}_2 \cdot \vec{v}_2 \hat{n} \cdot \vec{v}_1 + 16 \hat{n} \times \vec{S}_2 \cdot \vec{v}_1 \hat{n} \times \vec{S}_1 \cdot \vec{v}_1 \hat{n} \cdot \vec{v}_2 + \\ & 28 \hat{n} \times \vec{S}_1 \cdot \vec{v}_1 \hat{n} \times \vec{S}_2 \cdot \vec{a}_1 \hat{n} \cdot \vec{v}_2 + 12 \hat{n} \times \vec{S}_1 \cdot \vec{v}_1 \hat{n} \times \vec{S}_2 \cdot \vec{v}_1 \hat{n} \cdot \vec{v}_2 + 28 \hat{n} \times \vec{S}_1 \cdot \vec{a}_1 \hat{n} \times \vec{S}_2 \cdot \vec{v}_1 \hat{n} \cdot \vec{v}_2 + \\ & 4 \hat{n} \cdot \vec{S}_1 \hat{n} \cdot \vec{S}_2 \hat{n} \cdot \vec{v}_1 \vec{a}_1 \cdot \vec{v}_2 - \hat{n} \cdot \vec{v}_1 \vec{a}_1 \cdot \vec{v}_2 \vec{S}_1 \cdot \vec{S}_2 + 4 \hat{n} \cdot \vec{v}_2 \vec{S}_2 \cdot \vec{v}_1 \vec{S}_1 \cdot \vec{v}_1 + 2 \hat{n} \cdot \vec{v}_1 \vec{S}_2 \cdot \vec{v}_2 \vec{S}_1 \cdot \vec{v}_1 - \\ & \hat{n} \cdot \vec{S}_2 \vec{a}_1 \cdot \vec{v}_2 \vec{S}_1 \cdot \vec{v}_1 - 4 \hat{n} \cdot \vec{v}_1 \vec{S}_2 \cdot \vec{v}_1 \vec{S}_1 \cdot \vec{v}_2 + 7 \hat{n} \cdot \vec{v}_2 \vec{S}_1 \cdot \vec{v}_1 \vec{S}_2 \cdot \vec{a}_1 + 2 \hat{n} \cdot \vec{v}_1 \vec{S}_1 \cdot \vec{v}_2 \vec{S}_2 \cdot \vec{a}_1 + \\ & 2 \hat{n} \cdot \vec{v}_1 \vec{S}_1 \cdot \vec{v}_1 \vec{S}_2 \cdot \vec{a}_2 + 3 \hat{n} \cdot \vec{v}_2 \vec{S}_1 \cdot \vec{v}_1 \vec{S}_2 \cdot \vec{v}_1 - 6 \hat{n} \cdot \vec{v}_1 \vec{S}_1 \cdot \vec{v}_2 \vec{S}_2 \cdot \vec{v}_1 - \hat{n} \cdot \vec{S}_1 \vec{a}_1 \cdot \vec{v}_2 \vec{S}_2 \cdot \vec{v}_1 + \end{aligned}$$

$$\frac{1}{r^4}$$

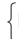

$$G^2 m_1 \left( 4 \vec{S}_1 \times \vec{v}_1 \cdot \vec{a}_1 \hat{n} \times \vec{S}_2 \cdot \vec{v}_1 - 8 \vec{S}_2 \times \vec{v}_1 \cdot \vec{a}_1 \hat{n} \times \vec{S}_1 \cdot \vec{v}_1 - 8 \hat{n} \cdot \vec{a}_1 \hat{n} \times \vec{S}_1 \cdot \vec{v}_1 \hat{n} \times \vec{S}_2 \cdot \vec{v}_1 - \right. \\ \left. 40 \hat{n} \cdot \vec{v}_1 \hat{n} \times \vec{S}_2 \cdot \vec{a}_1 \hat{n} \times \vec{S}_1 \cdot \vec{v}_1 + 8 \hat{n} \cdot \vec{v}_1 \hat{n} \times \vec{S}_1 \cdot \vec{a}_1 \hat{n} \times \vec{S}_2 \cdot \vec{v}_1 + 2 \vec{S}_2 \cdot \vec{a}_1 \hat{n} \cdot \vec{v}_1 \vec{S}_1 \cdot \vec{v}_1 - \right. \\ \left. 10 \vec{S}_1 \cdot \vec{a}_1 \hat{n} \cdot \vec{v}_1 \vec{S}_2 \cdot \vec{v}_1 - 2 \hat{n} \cdot \vec{a}_1 \vec{S}_1 \cdot \vec{v}_1 \vec{S}_2 \cdot \vec{v}_1 - 32 \vec{v}_1 \cdot \vec{a}_1 \hat{n} \cdot \vec{S}_1 \hat{n} \cdot \vec{S}_2 \hat{n} \cdot \vec{v}_1 + 10 \vec{S}_1 \cdot \vec{S}_2 \vec{v}_1 \cdot \vec{a}_1 \hat{n} \cdot \vec{v}_1 + \right. \\ \left. 8 \vec{v}_1 \cdot \vec{a}_1 \hat{n} \cdot \vec{S}_2 \vec{S}_1 \cdot \vec{v}_1 + 6 \vec{v}_1 \cdot \vec{a}_1 \hat{n} \cdot \vec{S}_1 \vec{S}_2 \cdot \vec{v}_1 - 8 \vec{v}_1 \cdot \vec{v}_1 \hat{n} \cdot \vec{a}_1 \hat{n} \cdot \vec{S}_1 \hat{n} \cdot \vec{S}_2 + 2 \vec{v}_1 \cdot \vec{v}_1 \vec{S}_1 \cdot \vec{a}_1 \hat{n} \cdot \vec{S}_2 + \right. \\ \left. 6 \vec{S}_1 \cdot \vec{S}_2 \vec{v}_1 \cdot \vec{v}_1 \hat{n} \cdot \vec{a}_1 - 2 \vec{v}_1 \cdot \vec{v}_1 \vec{S}_2 \cdot \vec{a}_1 \hat{n} \cdot \vec{S}_1 + 8 \hat{n} \cdot \vec{v}_1 \hat{n} \times \vec{S}_1 \cdot \vec{v}_1 \hat{n} \times \vec{S}_2 \cdot \vec{v}_1 + \right. \\ \left. 2 \hat{n} \cdot \vec{v}_1 \vec{S}_1 \cdot \vec{v}_1 \vec{S}_2 \cdot \vec{v}_1 + 8 \vec{v}_1 \cdot \vec{v}_1 \hat{n} \cdot \vec{S}_1 \hat{n} \cdot \vec{S}_2 \hat{n} \cdot \vec{v}_1 - 2 \vec{v}_1 \cdot \vec{v}_1 \hat{n} \cdot \vec{S}_2 \vec{S}_1 \cdot \vec{v}_1 - 4 \vec{v}_1 \cdot \vec{v}_1 \hat{n} \cdot \vec{S}_1 \vec{S}_2 \cdot \vec{v}_1 \right) \Bigg\}$$

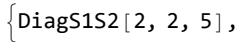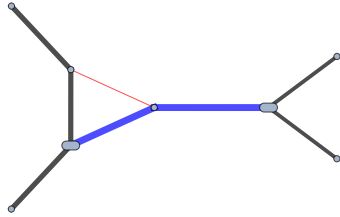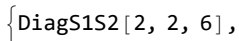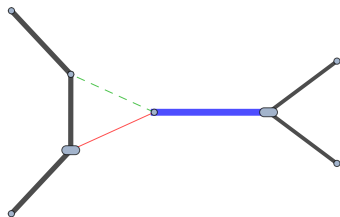

$$G^2 m_1 \left( \frac{1}{r^3} \left( -8 \vec{S}_1 \times \vec{a}_1 \cdot \vec{v}_2 \hat{n} \times \vec{S}_2 \cdot \vec{v}_1 + 8 \vec{S}_1 \times \vec{v}_1 \cdot \vec{v}_2 \hat{n} \times \vec{S}_2 \cdot \vec{a}_1 + 12 \vec{S}_2 \times \vec{a}_1 \cdot \vec{v}_2 \hat{n} \times \vec{S}_1 \cdot \vec{v}_1 - 4 \vec{S}_2 \times \vec{v}_1 \cdot \vec{v}_2 \hat{n} \times \vec{S}_1 \cdot \vec{a}_1 - \right. \right. \\ \left. \left. 48 \hat{n} \cdot \vec{v}_2 \hat{n} \times \vec{S}_2 \cdot \vec{a}_1 \hat{n} \times \vec{S}_1 \cdot \vec{v}_1 + 16 \hat{n} \cdot \vec{v}_2 \hat{n} \times \vec{S}_1 \cdot \vec{a}_1 \hat{n} \times \vec{S}_2 \cdot \vec{v}_1 + 4 \vec{S}_1 \cdot \vec{S}_2 \vec{a}_1 \cdot \vec{v}_2 \hat{n} \cdot \vec{v}_1 + 4 \vec{S}_2 \cdot \vec{a}_1 \hat{n} \cdot \vec{v}_2 \vec{S}_1 \cdot \vec{v}_1 - \right. \right. \\ \left. \left. 4 \vec{a}_1 \cdot \vec{v}_2 \hat{n} \cdot \vec{S}_1 \vec{S}_2 \cdot \vec{v}_1 - 12 \vec{S}_1 \cdot \vec{a}_1 \hat{n} \cdot \vec{v}_2 \vec{S}_2 \cdot \vec{v}_1 + 8 \vec{S}_1 \cdot \vec{S}_2 \vec{v}_1 \cdot \vec{a}_1 \hat{n} \cdot \vec{v}_2 + 4 \vec{S}_1 \cdot \vec{S}_2 \vec{v}_1 \cdot \vec{v}_2 \hat{n} \cdot \vec{a}_1 - \right. \right. \\ \left. \left. 4 \vec{S}_1 \cdot \vec{S}_2 \vec{v}_1 \cdot \vec{v}_2 \hat{n} \cdot \vec{a}_1 - 4 \vec{S}_1 \cdot \vec{S}_2 \vec{a}_1 \cdot \vec{v}_1 \hat{n} \cdot \vec{v}_2 + 4 \vec{S}_1 \cdot \vec{S}_2 \vec{a}_1 \cdot \vec{v}_1 \hat{n} \cdot \vec{v}_2 \right) \right)$$

$$\begin{aligned}
& 4 \vec{v}_1 \cdot \vec{v}_2 \vec{S}_2 \cdot \vec{a}_1 \hat{n} \cdot \vec{S}_1 - 8 \vec{S}_1 \times \vec{v}_1 \cdot \vec{v}_2 \hat{n} \times \vec{S}_2 \cdot \vec{v}_1 - 4 \vec{S}_2 \times \vec{v}_1 \cdot \vec{v}_2 \hat{n} \times \vec{S}_1 \cdot \vec{v}_1 + 16 \hat{n} \cdot \vec{v}_2 \hat{n} \times \vec{S}_1 \cdot \vec{v}_1 \hat{n} \times \vec{S}_2 \cdot \vec{v}_1 + \\
& 4 \hat{n} \cdot \vec{v}_2 \vec{S}_1 \cdot \vec{v}_1 \vec{S}_2 \cdot \vec{v}_1 - 4 \vec{S}_1 \cdot \vec{S}_2 \vec{v}_1 \cdot \vec{v}_1 \hat{n} \cdot \vec{v}_2 + 4 \vec{S}_1 \cdot \vec{S}_2 \vec{v}_1 \cdot \vec{v}_2 \hat{n} \cdot \vec{v}_1 - 4 \vec{v}_1 \cdot \vec{v}_2 \hat{n} \cdot \vec{S}_1 \vec{S}_2 \cdot \vec{v}_1 \Big) + \\
& \frac{1}{r^4} \Big( 16 \hat{n} \cdot \vec{v}_1 \vec{S}_1 \times \vec{v}_1 \cdot \vec{v}_2 \hat{n} \times \vec{S}_2 \cdot \vec{v}_1 - 16 \vec{S}_1 \cdot \vec{S}_2 \vec{v}_1 \cdot \vec{v}_2 (\hat{n} \cdot \vec{v}_1)^2 + 16 \vec{v}_1 \cdot \vec{v}_2 \hat{n} \cdot \vec{S}_1 \hat{n} \cdot \vec{v}_1 \vec{S}_2 \cdot \vec{v}_1 - \\
& 4 \vec{v}_1 \cdot \vec{v}_2 \vec{S}_1 \cdot \vec{v}_1 \vec{S}_2 \cdot \vec{v}_1 + 4 \vec{S}_1 \cdot \vec{S}_2 \vec{v}_1 \cdot \vec{v}_1 \vec{v}_1 \cdot \vec{v}_2 \Big) \Big) \Big\}
\end{aligned}$$

{DiagS1S2[2, 2, 7],

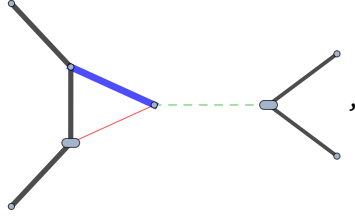

$$\begin{aligned}
& G^2 m_1 \left( \frac{1}{r^3} \left( -16 \vec{S}_1 \times \vec{v}_1 \cdot \vec{a}_1 \hat{n} \times \vec{S}_2 \cdot \vec{v}_1 - 64 \hat{n} \cdot \vec{v}_1 \hat{n} \times \vec{S}_1 \cdot \vec{a}_1 \hat{n} \times \vec{S}_2 \cdot \vec{v}_1 - 16 \vec{S}_2 \cdot \vec{a}_1 \hat{n} \cdot \vec{v}_1 \vec{S}_1 \cdot \vec{v}_1 + \right. \right. \\
& 16 \vec{S}_1 \cdot \vec{S}_2 \vec{v}_1 \cdot \vec{a}_1 \hat{n} \cdot \vec{v}_1 - 48 \hat{n} \cdot \vec{v}_1 \hat{n} \times \vec{S}_2 \cdot \vec{v}_1 \hat{n} \times \vec{S}_1 \cdot \vec{v}_1 - 64 \hat{n} \cdot \vec{v}_1 \hat{n} \times \vec{S}_1 \cdot \vec{v}_1 \hat{n} \times \vec{S}_2 \cdot \vec{v}_1 - \\
& 12 \hat{n} \cdot \vec{v}_1 \vec{S}_2 \cdot \vec{v}_1 \vec{S}_1 \cdot \vec{v}_1 - 16 \hat{n} \cdot \vec{v}_1 \vec{S}_1 \cdot \vec{v}_1 \vec{S}_2 \cdot \vec{v}_1 + 16 \vec{S}_1 \cdot \vec{S}_2 \vec{v}_1 \cdot \vec{v}_1 \hat{n} \cdot \vec{v}_1 + 12 \vec{S}_1 \cdot \vec{S}_2 \vec{v}_1 \cdot \vec{v}_1 \hat{n} \cdot \vec{v}_1 \Big) + \frac{1}{r^4} \\
& \left( 288 (\hat{n} \cdot \vec{v}_1)^2 \hat{n} \times \vec{S}_1 \cdot \vec{v}_1 \hat{n} \times \vec{S}_2 \cdot \vec{v}_1 + 48 \hat{n} \cdot \vec{v}_1 \vec{S}_1 \times \vec{v}_1 \cdot \vec{v}_2 \hat{n} \times \vec{S}_2 \cdot \vec{v}_1 + 48 \hat{n} \cdot \vec{v}_1 \vec{S}_2 \times \vec{v}_1 \cdot \vec{v}_2 \hat{n} \times \vec{S}_1 \cdot \vec{v}_1 - \right. \\
& 288 \hat{n} \cdot \vec{v}_2 \hat{n} \cdot \vec{v}_1 \hat{n} \times \vec{S}_1 \cdot \vec{v}_1 \hat{n} \times \vec{S}_2 \cdot \vec{v}_1 - 48 \vec{v}_1 \cdot \vec{v}_1 \hat{n} \times \vec{S}_1 \cdot \vec{v}_1 \hat{n} \times \vec{S}_2 \cdot \vec{v}_1 + 48 \vec{v}_1 \cdot \vec{v}_2 \hat{n} \times \vec{S}_1 \cdot \vec{v}_1 \hat{n} \times \vec{S}_2 \cdot \vec{v}_1 + \\
& 48 (\hat{n} \cdot \vec{v}_1)^2 \vec{S}_1 \cdot \vec{v}_1 \vec{S}_2 \cdot \vec{v}_1 - 48 \vec{S}_1 \cdot \vec{S}_2 \vec{v}_1 \cdot \vec{v}_1 (\hat{n} \cdot \vec{v}_1)^2 - 48 \hat{n} \cdot \vec{v}_2 \hat{n} \cdot \vec{v}_1 \vec{S}_1 \cdot \vec{v}_1 \vec{S}_2 \cdot \vec{v}_1 + 48 \vec{S}_1 \cdot \vec{S}_2 \vec{v}_1 \cdot \vec{v}_1 \hat{n} \cdot \vec{v}_2 \\
& \left. \hat{n} \cdot \vec{v}_1 + 12 \vec{S}_1 \cdot \vec{S}_2 (\vec{v}_1 \cdot \vec{v}_1)^2 - 12 \vec{v}_1 \cdot \vec{v}_1 \vec{S}_1 \cdot \vec{v}_1 \vec{S}_2 \cdot \vec{v}_1 + 12 \vec{v}_1 \cdot \vec{v}_2 \vec{S}_1 \cdot \vec{v}_1 \vec{S}_2 \cdot \vec{v}_1 - 12 \vec{S}_1 \cdot \vec{S}_2 \vec{v}_1 \cdot \vec{v}_1 \vec{v}_1 \cdot \vec{v}_2 \right) \Big) \Big\}
\end{aligned}$$

{DiagS1S2[2, 2, 8],

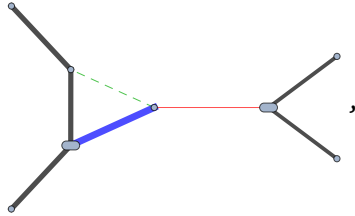

$$\begin{aligned}
& G^2 \left( \frac{1}{r^3} \left( 4 \hat{n} \times \vec{S}_1 \cdot \vec{v}_1 \vec{S}_2 \times \vec{v}_1 \cdot \vec{v}_2 + 16 \hat{n} \times \vec{S}_2 \cdot \vec{v}_2 \vec{S}_1 \times \vec{v}_1 \cdot \vec{a}_1 + 4 \hat{n} \times \vec{S}_1 \cdot \vec{v}_1 \vec{S}_2 \times \vec{v}_1 \cdot \vec{a}_2 + \right. \right. \\
& 16 \hat{n} \times \vec{S}_1 \cdot \vec{a}_1 \vec{S}_2 \times \vec{v}_1 \cdot \vec{v}_2 + 16 \hat{n} \times \vec{S}_2 \cdot \vec{v}_2 \hat{n} \times \vec{S}_1 \cdot \vec{v}_1 \hat{n} \cdot \vec{v}_1 + 16 \hat{n} \times \vec{S}_1 \cdot \vec{v}_1 \hat{n} \times \vec{S}_2 \cdot \vec{a}_2 \hat{n} \cdot \vec{v}_1 + \\
& 64 \hat{n} \times \vec{S}_1 \cdot \vec{a}_1 \hat{n} \times \vec{S}_2 \cdot \vec{v}_2 \hat{n} \cdot \vec{v}_1 - 16 \hat{n} \cdot \vec{v}_1 \vec{a}_1 \cdot \vec{v}_2 \vec{S}_1 \cdot \vec{S}_2 + 4 \hat{n} \cdot \vec{v}_1 \vec{S}_2 \cdot \vec{v}_1 \vec{S}_1 \cdot \vec{v}_2 + \\
& 16 \hat{n} \cdot \vec{v}_1 \vec{S}_1 \cdot \vec{v}_2 \vec{S}_2 \cdot \vec{a}_1 + 4 \hat{n} \cdot \vec{v}_1 \vec{S}_1 \cdot \vec{a}_2 \vec{S}_2 \cdot \vec{v}_1 - 4 \hat{n} \cdot \vec{v}_1 \vec{S}_1 \cdot \vec{S}_2 \vec{v}_1 \cdot \vec{a}_2 - 4 \hat{n} \cdot \vec{v}_1 \vec{S}_1 \cdot \vec{S}_2 \vec{v}_1 \cdot \vec{v}_2 \Big) + \\
& \frac{1}{r^4} \left( -96 \hat{n} \times \vec{S}_1 \cdot \vec{v}_1 \hat{n} \times \vec{S}_2 \cdot \vec{v}_2 (\hat{n} \cdot \vec{v}_1)^2 - 16 \vec{S}_1 \cdot \vec{v}_2 \vec{S}_2 \cdot \vec{v}_1 (\hat{n} \cdot \vec{v}_1)^2 + 16 \vec{S}_1 \cdot \vec{S}_2 \vec{v}_1 \cdot \vec{v}_2 (\hat{n} \cdot \vec{v}_1)^2 - \right. \\
& 16 \hat{n} \times \vec{S}_2 \cdot \vec{v}_2 \vec{S}_1 \times \vec{v}_1 \cdot \vec{v}_2 \hat{n} \cdot \vec{v}_1 - 32 \hat{n} \times \vec{S}_1 \cdot \vec{v}_1 \vec{S}_2 \times \vec{v}_1 \cdot \vec{v}_2 \hat{n} \cdot \vec{v}_1 + 96 \hat{n} \times \vec{S}_1 \cdot \vec{v}_1 \hat{n} \times \vec{S}_2 \cdot \vec{v}_2 \hat{n} \cdot \vec{v}_2 \hat{n} \cdot \vec{v}_1 + \\
& 16 \hat{n} \cdot \vec{v}_2 \vec{S}_1 \cdot \vec{v}_2 \vec{S}_2 \cdot \vec{v}_1 \hat{n} \cdot \vec{v}_1 - 16 \hat{n} \cdot \vec{v}_2 \vec{S}_1 \cdot \vec{S}_2 \vec{v}_1 \cdot \vec{v}_2 \hat{n} \cdot \vec{v}_1 + 4 \vec{S}_1 \cdot \vec{S}_2 (\vec{v}_1 \cdot \vec{v}_2)^2 - 4 \vec{S}_1 \times \vec{v}_1 \cdot \vec{v}_2 \vec{S}_2 \times \vec{v}_1 \cdot \vec{v}_2 + \\
& \left. 16 \hat{n} \times \vec{S}_1 \cdot \vec{v}_1 \vec{S}_2 \times \vec{v}_1 \cdot \vec{v}_2 \hat{n} \cdot \vec{v}_2 - 16 \hat{n} \times \vec{S}_1 \cdot \vec{v}_1 \hat{n} \times \vec{S}_2 \cdot \vec{v}_2 \vec{v}_1 \cdot \vec{v}_2 - 4 \vec{S}_1 \cdot \vec{v}_2 \vec{S}_2 \cdot \vec{v}_1 \vec{v}_1 \cdot \vec{v}_2 \right) \Big) m_1 \Big\}
\end{aligned}$$



$$\{\text{DiagS1S2}[2, 2, 9],$$

$$\frac{1}{r^4} \left( -288 \hat{n} \cdot \vec{S}_1 \cdot \vec{v}_1 \hat{n} \cdot \vec{S}_2 \cdot \vec{v}_2 (\hat{n} \cdot \vec{v}_1)^2 - 48 \vec{S}_1 \cdot \vec{v}_2 \vec{S}_2 \cdot \vec{v}_1 (\hat{n} \cdot \vec{v}_1)^2 + 48 \vec{S}_1 \cdot \vec{S}_2 \vec{v}_1 \cdot \vec{v}_2 (\hat{n} \cdot \vec{v}_1)^2 - \right.$$

$$\{\text{DiagS1S2}[2, 2, 10],$$

$$G^2 m_1 \left( 288 \left( \hat{n} \cdot \vec{v}_1 \right)^2 \hat{n} \times \vec{S}_1 \cdot \vec{v}_1 \hat{n} \times \vec{S}_2 \cdot \vec{v}_2 + 96 \hat{n} \cdot \vec{v}_1 \vec{S}_2 \times \vec{v}_1 \cdot \vec{v}_2 \hat{n} \times \vec{S}_1 \cdot \vec{v}_1 - 48 \vec{v}_1 \cdot \vec{v}_1 \hat{n} \times \vec{S}_1 \cdot \vec{v}_1 \hat{n} \times \vec{S}_2 \cdot \vec{v}_2 + \right. \\ \left. 48 \left( \hat{n} \cdot \vec{v}_1 \right)^2 \vec{S}_1 \cdot \vec{v}_2 \vec{S}_2 \cdot \vec{v}_1 - 48 \vec{S}_1 \cdot \vec{S}_2 \vec{v}_1 \cdot \vec{v}_2 \left( \hat{n} \cdot \vec{v}_1 \right)^2 - 12 \vec{v}_1 \cdot \vec{v}_1 \vec{S}_1 \cdot \vec{v}_2 \vec{S}_2 \cdot \vec{v}_1 + 12 \vec{S}_1 \cdot \vec{S}_2 \vec{v}_1 \cdot \vec{v}_1 \vec{v}_1 \cdot \vec{v}_2 \right) \Big\}$$

$$\{\text{DiagS1S2}[2, 2, 11],$$

$$G^2 \left( \frac{1}{r^3} \left( -12 \hat{n} \times \vec{S}_1 \cdot \vec{v}_1 \vec{S}_2 \times \vec{v}_1 \cdot \vec{v}_2 + 16 \hat{n} \times \vec{S}_2 \cdot \vec{v}_2 \vec{S}_1 \times \vec{v}_1 \cdot \vec{a}_1 - 12 \hat{n} \times \vec{S}_1 \cdot \vec{v}_1 \vec{S}_2 \times \vec{v}_1 \cdot \vec{a}_2 + \right. \right.$$

$$\frac{1}{r^4} \left( -288 \hat{n} \cdot \vec{S}_1 \cdot \vec{v}_1 \hat{n} \cdot \vec{S}_2 \cdot \vec{v}_2 (\hat{n} \cdot \vec{v}_1)^2 - 48 \vec{S}_1 \cdot \vec{v}_2 \vec{S}_2 \cdot \vec{v}_1 (\hat{n} \cdot \vec{v}_1)^2 + 48 \vec{S}_1 \cdot \vec{S}_2 \vec{v}_1 \cdot \vec{v}_2 (\hat{n} \cdot \vec{v}_1)^2 + \right.$$

$$\left. 48 \hat{n} \times \vec{S}_1 \cdot \vec{v}_1 \hat{n} \times \vec{S}_2 \cdot \vec{v}_2 \vec{v}_1 \cdot \vec{v}_2 + 12 \vec{S}_1 \cdot \vec{v}_2 \vec{S}_2 \cdot \vec{v}_1 \vec{v}_1 \cdot \vec{v}_2 - 12 \vec{S}_1 \cdot \vec{S}_2 \vec{v}_1 \cdot \vec{v}_1 \vec{v}_1 \cdot \vec{v}_2 \right) \bigg) m_1 \bigg\}$$

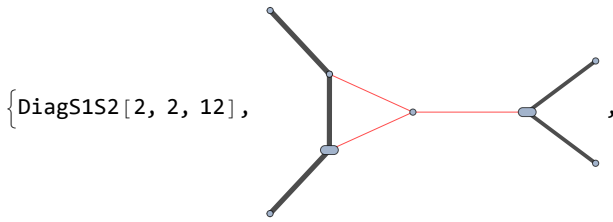

$$G^2 \left( \frac{1}{r^2} \left( -16 \hat{n} \times \vec{S}_1 \cdot \vec{v}_1 \hat{n} \times \vec{S}_2 \cdot \vec{v}_2 - 16 \hat{n} \times \vec{S}_1 \cdot \vec{a}_1 \hat{n} \times \vec{S}_2 \cdot \vec{v}_2 - 16 \hat{n} \times \vec{S}_1 \cdot \vec{v}_1 \hat{n} \times \vec{S}_2 \cdot \vec{a}_2 - \right. \right. \\ \left. \left. 16 \hat{n} \times \vec{S}_1 \cdot \vec{a}_1 \hat{n} \times \vec{S}_2 \cdot \vec{a}_2 - 8 \vec{S}_1 \cdot \vec{v}_2 \vec{S}_2 \cdot \vec{v}_1 + 8 \vec{a}_1 \cdot \vec{v}_2 \vec{S}_1 \cdot \vec{S}_2 + 8 \vec{a}_1 \cdot \vec{a}_2 \vec{S}_1 \cdot \vec{S}_2 - \right. \right. \\ \left. \left. 8 \vec{S}_2 \cdot \vec{a}_1 \vec{S}_1 \cdot \vec{v}_2 - 8 \vec{S}_1 \cdot \vec{a}_2 \vec{S}_2 \cdot \vec{a}_1 - 8 \vec{S}_1 \cdot \vec{a}_2 \vec{S}_2 \cdot \vec{v}_1 + 8 \vec{S}_1 \cdot \vec{S}_2 \vec{v}_1 \cdot \vec{a}_2 + 8 \vec{S}_1 \cdot \vec{S}_2 \vec{v}_1 \cdot \vec{v}_2 \right) + \frac{1}{r^3} \right. \\ \left. \left( 16 \hat{n} \times \vec{S}_2 \cdot \vec{v}_2 \vec{S}_1 \times \vec{v}_1 \cdot \vec{v}_2 + 16 \hat{n} \times \vec{S}_1 \cdot \vec{v}_1 \vec{S}_2 \times \vec{v}_1 \cdot \vec{v}_2 + 16 \hat{n} \times \vec{S}_2 \cdot \vec{v}_2 \vec{S}_1 \times \vec{a}_1 \cdot \vec{v}_2 + 8 \hat{n} \times \vec{S}_2 \cdot \vec{v}_2 \vec{S}_1 \times \vec{v}_1 \cdot \vec{a}_1 + \right. \right. \\ \left. \left. 16 \hat{n} \times \vec{S}_1 \cdot \vec{v}_1 \vec{S}_2 \times \vec{v}_1 \cdot \vec{a}_2 + 4 \hat{n} \times \vec{S}_1 \cdot \vec{v}_1 \vec{S}_2 \times \vec{v}_1 \cdot \vec{v}_2 + 4 \hat{n} \times \vec{S}_1 \cdot \vec{a}_1 \vec{S}_2 \times \vec{v}_1 \cdot \vec{v}_2 + \right. \right. \\ \left. \left. 64 \hat{n} \times \vec{S}_2 \cdot \vec{v}_2 \hat{n} \times \vec{S}_1 \cdot \vec{v}_1 \hat{n} \cdot \vec{v}_1 + 64 \hat{n} \times \vec{S}_1 \cdot \vec{v}_1 \hat{n} \times \vec{S}_2 \cdot \vec{a}_2 \hat{n} \cdot \vec{v}_1 + 16 \hat{n} \times \vec{S}_1 \cdot \vec{v}_1 \hat{n} \times \vec{S}_2 \cdot \vec{v}_2 \hat{n} \cdot \vec{v}_1 + \right. \right. \\ \left. \left. 16 \hat{n} \times \vec{S}_1 \cdot \vec{a}_1 \hat{n} \times \vec{S}_2 \cdot \vec{v}_2 \hat{n} \cdot \vec{v}_1 - 64 \hat{n} \times \vec{S}_1 \cdot \vec{v}_1 \hat{n} \times \vec{S}_2 \cdot \vec{v}_2 \hat{n} \cdot \vec{v}_2 - 64 \hat{n} \times \vec{S}_1 \cdot \vec{a}_1 \hat{n} \times \vec{S}_2 \cdot \vec{v}_2 \hat{n} \cdot \vec{v}_2 - \right. \right. \\ \left. \left. 4 \hat{n} \cdot \vec{v}_1 \vec{a}_1 \cdot \vec{v}_2 \vec{S}_1 \cdot \vec{S}_2 + 16 \hat{n} \cdot \vec{v}_2 \vec{a}_1 \cdot \vec{v}_2 \vec{S}_1 \cdot \vec{S}_2 + 16 \hat{n} \cdot \vec{v}_1 \vec{S}_2 \cdot \vec{v}_1 \vec{S}_1 \cdot \vec{v}_2 + 4 \hat{n} \cdot \vec{v}_1 \vec{S}_1 \cdot \vec{v}_2 \vec{S}_2 \cdot \vec{a}_1 - \right. \right. \\ \left. \left. 16 \hat{n} \cdot \vec{v}_2 \vec{S}_1 \cdot \vec{v}_2 \vec{S}_2 \cdot \vec{a}_1 + 4 \hat{n} \cdot \vec{v}_1 \vec{S}_1 \cdot \vec{v}_2 \vec{S}_2 \cdot \vec{v}_1 - 16 \hat{n} \cdot \vec{v}_2 \vec{S}_1 \cdot \vec{v}_2 \vec{S}_2 \cdot \vec{v}_1 + 16 \hat{n} \cdot \vec{v}_1 \vec{S}_1 \cdot \vec{a}_2 \vec{S}_2 \cdot \vec{v}_1 - \right. \right. \\ \left. \left. 16 \hat{n} \cdot \vec{v}_1 \vec{S}_1 \cdot \vec{S}_2 \vec{v}_1 \cdot \vec{a}_2 - 4 \hat{n} \cdot \vec{v}_1 \vec{S}_1 \cdot \vec{S}_2 \vec{v}_1 \cdot \vec{v}_2 + 16 \hat{n} \cdot \vec{v}_2 \vec{S}_1 \cdot \vec{S}_2 \vec{v}_1 \cdot \vec{v}_2 - 16 \hat{n} \cdot \vec{v}_1 \vec{S}_1 \cdot \vec{S}_2 \vec{v}_1 \cdot \vec{v}_2 \right) + \right. \\ \left. \frac{1}{r^4} \left( -48 \hat{n} \times \vec{S}_1 \cdot \vec{v}_1 \hat{n} \times \vec{S}_2 \cdot \vec{v}_2 (\hat{n} \cdot \vec{v}_1)^2 - 8 \vec{S}_1 \cdot \vec{v}_2 \vec{S}_2 \cdot \vec{v}_1 (\hat{n} \cdot \vec{v}_1)^2 + 8 \vec{S}_1 \cdot \vec{S}_2 \vec{v}_1 \cdot \vec{v}_2 (\hat{n} \cdot \vec{v}_1)^2 - \right. \right. \\ \left. \left. 64 \hat{n} \times \vec{S}_2 \cdot \vec{v}_2 \vec{S}_1 \times \vec{v}_1 \cdot \vec{v}_2 \hat{n} \cdot \vec{v}_1 - 16 \hat{n} \times \vec{S}_1 \cdot \vec{v}_1 \vec{S}_2 \times \vec{v}_1 \cdot \vec{v}_2 \hat{n} \cdot \vec{v}_1 + 384 \hat{n} \times \vec{S}_1 \cdot \vec{v}_1 \hat{n} \times \vec{S}_2 \cdot \vec{v}_2 \hat{n} \cdot \vec{v}_2 \hat{n} \cdot \vec{v}_1 + \right. \right. \\ \left. \left. 64 \hat{n} \cdot \vec{v}_2 \vec{S}_1 \cdot \vec{v}_2 \vec{S}_2 \cdot \vec{v}_1 \hat{n} \cdot \vec{v}_1 - 64 \hat{n} \cdot \vec{v}_2 \vec{S}_1 \cdot \vec{S}_2 \vec{v}_1 \cdot \vec{v}_2 \hat{n} \cdot \vec{v}_1 + 16 \vec{S}_1 \cdot \vec{S}_2 (\vec{v}_1 \cdot \vec{v}_2)^2 - 16 \vec{S}_1 \times \vec{v}_1 \cdot \vec{v}_2 \vec{S}_2 \times \vec{v}_1 \cdot \vec{v}_2 + \right. \right. \\ \left. \left. 64 \hat{n} \times \vec{S}_1 \cdot \vec{v}_1 \vec{S}_2 \times \vec{v}_1 \cdot \vec{v}_2 \hat{n} \cdot \vec{v}_2 + 16 \hat{n} \times \vec{S}_1 \cdot \vec{v}_1 \hat{n} \times \vec{S}_2 \cdot \vec{v}_2 \vec{v}_1 \cdot \vec{v}_1 + 4 \vec{S}_1 \cdot \vec{v}_2 \vec{S}_2 \cdot \vec{v}_1 \vec{v}_1 \cdot \vec{v}_1 - \right. \right. \\ \left. \left. 64 \hat{n} \times \vec{S}_1 \cdot \vec{v}_1 \hat{n} \times \vec{S}_2 \cdot \vec{v}_2 \vec{v}_1 \cdot \vec{v}_2 - 16 \vec{S}_1 \cdot \vec{v}_2 \vec{S}_2 \cdot \vec{v}_1 \vec{v}_1 \cdot \vec{v}_2 - 4 \vec{S}_1 \cdot \vec{S}_2 \vec{v}_1 \cdot \vec{v}_1 \vec{v}_1 \cdot \vec{v}_2 \right) \right) m_1 \} \\$$

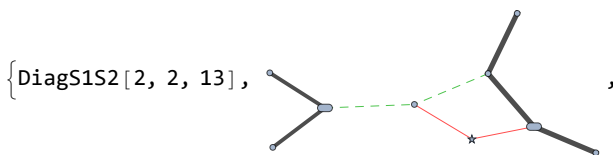

$$\begin{aligned} G^2 \left( \frac{1}{r^2} \right. & \left( -8 \vec{S_1} \cdot \vec{S_2} (\hat{n} \cdot \vec{a_1})^2 - 8 \hat{n} \cdot \vec{v_1} \vec{S_1} \cdot \vec{S_2} \hat{n} \cdot \vec{a_1} - 8 \hat{n} \cdot \vec{v_1} \vec{S_1} \cdot \vec{S_2} \hat{n} \cdot \vec{a_1} + 8 \hat{n} \cdot \vec{S_1} \vec{S_2} \cdot \vec{a_1} \hat{n} \cdot \vec{a_1} + 8 \hat{n} \cdot \vec{S_1} \vec{S_2} \cdot \vec{v_1} \hat{n} \cdot \vec{a_1} - \right. \\ & 8 (\hat{n} \cdot \vec{v_1})^2 \vec{S_1} \cdot \vec{S_2} + 8 \hat{n} \cdot \vec{S_1} \hat{n} \cdot \vec{v_1} \vec{S_2} \cdot \vec{a_1} + 8 \hat{n} \cdot \vec{S_1} \hat{n} \cdot \vec{v_1} \vec{S_2} \cdot \vec{v_1} - 4 \vec{S_1} \cdot \vec{v_1} \vec{S_2} \cdot \vec{v_1} + 4 \vec{a_1} \cdot \vec{a_1} \vec{S_1} \cdot \vec{S_2} - \\ & \left. 4 \vec{S_2} \cdot \vec{a_1} \vec{S_1} \cdot \vec{v_1} - 4 \vec{S_1} \cdot \vec{a_1} \vec{S_2} \cdot \vec{a_1} - 4 \vec{S_1} \cdot \vec{a_1} \vec{S_2} \cdot \vec{v_1} + 4 \vec{S_1} \cdot \vec{S_2} \vec{v_1} \cdot \vec{a_1} + 4 \vec{S_1} \cdot \vec{S_2} \vec{v_1} \cdot \vec{a_1} + 4 \vec{S_1} \cdot \vec{S_2} \vec{v_1} \cdot \vec{v_1} \right) + \\ & \left. \frac{1}{r^3} \left( 24 \vec{S_1} \cdot \vec{S_2} (\hat{n} \cdot \vec{v_1})^3 + 8 \vec{S_1} \cdot \vec{S_2} (\hat{n} \cdot \vec{v_1})^3 - 32 \hat{n} \cdot \vec{v_2} \vec{S_1} \cdot \vec{S_2} (\hat{n} \cdot \vec{v_1})^2 - 8 \hat{n} \cdot \vec{S_1} \vec{S_2} \cdot \vec{v_1} (\hat{n} \cdot \vec{v_1})^2 + \right. \right. \\ & 32 \hat{n} \cdot \vec{a_1} \vec{S_1} \cdot \vec{S_2} (\hat{n} \cdot \vec{v_1})^2 - 24 \hat{n} \cdot \vec{S_1} \vec{S_2} \cdot \vec{a_1} (\hat{n} \cdot \vec{v_1})^2 - 24 \hat{n} \cdot \vec{S_1} \vec{S_2} \cdot \vec{v_1} (\hat{n} \cdot \vec{v_1})^2 + \\ & 8 \hat{n} \times \vec{S_1} \cdot \vec{v_1} \hat{n} \times \vec{S_2} \cdot \vec{a_1} \hat{n} \cdot \vec{v_1} - 32 \hat{n} \cdot \vec{a_1} \hat{n} \cdot \vec{v_2} \vec{S_1} \cdot \vec{S_2} \hat{n} \cdot \vec{v_1} + 8 \vec{a_1} \cdot \vec{v_2} \vec{S_1} \cdot \vec{S_2} \hat{n} \cdot \vec{v_1} + \\ & \left. 4 \vec{S_2} \cdot \vec{v_1} \vec{S_1} \cdot \vec{v_1} \hat{n} \cdot \vec{v_1} + 32 \hat{n} \cdot \vec{S_1} \hat{n} \cdot \vec{v_2} \vec{S_2} \cdot \vec{a_1} \hat{n} \cdot \vec{v_1} + 12 \vec{S_1} \cdot \vec{v_1} \vec{S_2} \cdot \vec{a_1} \hat{n} \cdot \vec{v_1} - 8 \vec{S_1} \cdot \vec{v_2} \vec{S_2} \cdot \vec{a_1} \hat{n} \cdot \vec{v_1} - \right. \end{aligned}$$



{DiagS1S2[2, 2, 15],

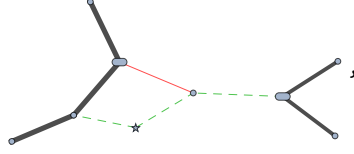

$$\begin{aligned}
 G^2 \left( \frac{1}{r^2} \left( -8 \vec{S}_1 \cdot \vec{S}_2 (\hat{n} \cdot \vec{a}_1)^2 - 8 \hat{n} \cdot \vec{v}_1 \vec{S}_1 \cdot \vec{S}_2 \hat{n} \cdot \vec{a}_1 + 8 \hat{n} \cdot \vec{S}_1 \vec{S}_2 \cdot \vec{v}_1 \hat{n} \cdot \vec{a}_1 - \right. \right. \\
 8 \hat{n} \cdot \vec{v}_1 \vec{S}_1 \cdot \vec{S}_2 \hat{n} \cdot \vec{a}_1 + 8 \hat{n} \cdot \vec{S}_1 \vec{S}_2 \cdot \vec{a}_1 \hat{n} \cdot \vec{a}_1 + 8 \hat{n} \cdot \vec{S}_1 \vec{S}_2 \cdot \vec{v}_1 \hat{n} \cdot \vec{a}_1 - 4 \vec{S}_2 \cdot \vec{v}_1 \vec{S}_1 \cdot \vec{a}_1 + \\
 4 \vec{a}_1 \cdot \vec{a}_1 \vec{S}_1 \cdot \vec{S}_2 - 4 \vec{S}_1 \cdot \vec{a}_1 \vec{S}_2 \cdot \vec{a}_1 - 4 \vec{S}_1 \cdot \vec{a}_1 \vec{S}_2 \cdot \vec{v}_1 + 4 \vec{S}_1 \cdot \vec{S}_2 \vec{v}_1 \cdot \vec{a}_1 + 4 \vec{S}_1 \cdot \vec{S}_2 \vec{v}_1 \cdot \vec{a}_1 \Big) + \frac{1}{r^3} \\
 \left( 8 \vec{S}_1 \cdot \vec{S}_2 (\hat{n} \cdot \vec{v}_1)^3 + 8 \vec{S}_1 \cdot \vec{S}_2 (\hat{n} \cdot \vec{v}_1)^3 - 8 \hat{n} \cdot \vec{S}_1 \vec{S}_2 \cdot \vec{v}_1 (\hat{n} \cdot \vec{v}_1)^2 + 32 \hat{n} \cdot \vec{a}_1 \vec{S}_1 \cdot \vec{S}_2 (\hat{n} \cdot \vec{v}_1)^2 - \right. \\
 8 \hat{n} \cdot \vec{S}_1 \vec{S}_2 \cdot \vec{a}_1 (\hat{n} \cdot \vec{v}_1)^2 - 8 \hat{n} \cdot \vec{S}_1 \vec{S}_2 \cdot \vec{v}_1 (\hat{n} \cdot \vec{v}_1)^2 + 24 \hat{n} \times \vec{S}_1 \cdot \vec{v}_1 \hat{n} \times \vec{S}_2 \cdot \vec{a}_1 \hat{n} \cdot \vec{v}_1 - \\
 32 \hat{n} \cdot \vec{a}_1 \hat{n} \cdot \vec{v}_2 \vec{S}_1 \cdot \vec{S}_2 \hat{n} \cdot \vec{v}_1 + 8 \vec{a}_1 \cdot \vec{v}_2 \vec{S}_1 \cdot \vec{S}_2 \hat{n} \cdot \vec{v}_1 + 4 \vec{S}_2 \cdot \vec{v}_1 \vec{S}_1 \cdot \vec{v}_1 \hat{n} \cdot \vec{v}_1 + 4 \vec{S}_1 \cdot \vec{v}_1 \vec{S}_2 \cdot \vec{a}_1 \hat{n} \cdot \vec{v}_1 - \\
 24 \hat{n} \cdot \vec{a}_1 \hat{n} \cdot \vec{S}_1 \vec{S}_2 \cdot \vec{v}_1 \hat{n} \cdot \vec{v}_1 + 4 \vec{S}_1 \cdot \vec{v}_1 \vec{S}_2 \cdot \vec{v}_1 \hat{n} \cdot \vec{v}_1 + 12 \vec{S}_1 \cdot \vec{a}_1 \vec{S}_2 \cdot \vec{v}_1 \hat{n} \cdot \vec{v}_1 - 22 \vec{S}_1 \cdot \vec{S}_2 \vec{v}_1 \cdot \vec{a}_1 \hat{n} \cdot \vec{v}_1 - \\
 6 \vec{S}_1 \cdot \vec{S}_2 \vec{v}_1 \cdot \vec{v}_1 \hat{n} \cdot \vec{v}_1 - 6 \vec{S}_1 \cdot \vec{S}_2 \vec{v}_1 \cdot \vec{v}_1 \hat{n} \cdot \vec{v}_1 + 8 \hat{n} \times \vec{S}_2 \cdot \vec{v}_1 \vec{S}_1 \times \vec{v}_1 \cdot \vec{a}_1 + 12 \hat{n} \times \vec{S}_1 \cdot \vec{v}_1 \vec{S}_2 \times \vec{v}_1 \cdot \vec{a}_1 - \\
 24 \hat{n} \times \vec{S}_1 \cdot \vec{v}_1 \hat{n} \times \vec{S}_2 \cdot \vec{v}_1 \hat{n} \cdot \vec{a}_1 + 32 \hat{n} \cdot \vec{a}_1 \hat{n} \cdot \vec{S}_1 \hat{n} \cdot \vec{v}_2 \vec{S}_2 \cdot \vec{v}_1 - 8 \hat{n} \cdot \vec{S}_1 \vec{a}_1 \cdot \vec{v}_2 \vec{S}_2 \cdot \vec{v}_1 - 8 \hat{n} \cdot \vec{v}_2 \vec{S}_1 \cdot \vec{a}_1 \vec{S}_2 \cdot \vec{v}_1 - \\
 8 \hat{n} \cdot \vec{a}_1 \vec{S}_1 \cdot \vec{v}_2 \vec{S}_2 \cdot \vec{v}_1 + 8 \hat{n} \cdot \vec{v}_2 \vec{S}_1 \cdot \vec{S}_2 \vec{v}_1 \cdot \vec{a}_1 + 6 \hat{n} \cdot \vec{S}_1 \vec{S}_2 \cdot \vec{v}_1 \vec{v}_1 \cdot \vec{a}_1 + 2 \hat{n} \cdot \vec{S}_1 \vec{S}_2 \cdot \vec{v}_1 \vec{v}_1 \cdot \vec{v}_1 - \\
 2 \hat{n} \cdot \vec{a}_1 \vec{S}_1 \cdot \vec{S}_2 \vec{v}_1 \cdot \vec{v}_1 + 2 \hat{n} \cdot \vec{S}_1 \vec{S}_2 \cdot \vec{a}_1 \vec{v}_1 \cdot \vec{v}_1 + 2 \hat{n} \cdot \vec{S}_1 \vec{S}_2 \cdot \vec{v}_1 \vec{v}_1 \cdot \vec{v}_1 + 8 \hat{n} \cdot \vec{a}_1 \vec{S}_1 \cdot \vec{S}_2 \vec{v}_1 \cdot \vec{v}_2 \Big) + \frac{1}{r^4} \\
 \left( -24 \vec{S}_1 \cdot \vec{S}_2 (\hat{n} \cdot \vec{v}_1)^4 + 48 \hat{n} \cdot \vec{v}_2 \vec{S}_1 \cdot \vec{S}_2 (\hat{n} \cdot \vec{v}_1)^3 + 24 \hat{n} \cdot \vec{S}_1 \vec{S}_2 \cdot \vec{v}_1 (\hat{n} \cdot \vec{v}_1)^3 - 48 \hat{n} \cdot \vec{S}_1 \hat{n} \cdot \vec{v}_2 \vec{S}_2 \cdot \vec{v}_1 (\hat{n} \cdot \vec{v}_1)^2 - \right. \\
 12 \vec{S}_1 \cdot \vec{v}_1 \vec{S}_2 \cdot \vec{v}_1 (\hat{n} \cdot \vec{v}_1)^2 + 8 \vec{S}_1 \cdot \vec{v}_2 \vec{S}_2 \cdot \vec{v}_1 (\hat{n} \cdot \vec{v}_1)^2 + 28 \vec{S}_1 \cdot \vec{S}_2 \vec{v}_1 \cdot \vec{v}_1 (\hat{n} \cdot \vec{v}_1)^2 - 24 \vec{S}_1 \cdot \vec{S}_2 \vec{v}_1 \cdot \vec{v}_2 (\hat{n} \cdot \vec{v}_1)^2 + \\
 16 \hat{n} \cdot \vec{v}_2 \vec{S}_1 \cdot \vec{v}_1 \vec{S}_2 \cdot \vec{v}_1 \hat{n} \cdot \vec{v}_1 - 24 \hat{n} \cdot \vec{v}_2 \vec{S}_1 \cdot \vec{S}_2 \vec{v}_1 \cdot \vec{v}_1 \hat{n} \cdot \vec{v}_1 - 16 \hat{n} \cdot \vec{S}_1 \vec{S}_2 \cdot \vec{v}_1 \vec{v}_1 \cdot \vec{v}_1 \hat{n} \cdot \vec{v}_1 + \\
 16 \hat{n} \cdot \vec{S}_1 \vec{S}_2 \cdot \vec{v}_1 \vec{v}_1 \cdot \vec{v}_2 \hat{n} \cdot \vec{v}_1 - 6 \vec{S}_1 \cdot \vec{S}_2 (\vec{v}_1 \cdot \vec{v}_1)^2 + 8 \hat{n} \times \vec{S}_1 \cdot \vec{v}_1 \hat{n} \times \vec{S}_2 \cdot \vec{v}_1 \vec{v}_1 \cdot \vec{v}_1 + 8 \hat{n} \cdot \vec{S}_1 \hat{n} \cdot \vec{v}_2 \vec{S}_2 \cdot \vec{v}_1 \vec{v}_1 \cdot \vec{v}_1 + \\
 6 \vec{S}_1 \cdot \vec{v}_1 \vec{S}_2 \cdot \vec{v}_1 \vec{v}_1 \cdot \vec{v}_1 - 2 \vec{S}_1 \cdot \vec{v}_2 \vec{S}_2 \cdot \vec{v}_1 \vec{v}_1 \cdot \vec{v}_1 - 4 \vec{S}_1 \cdot \vec{v}_1 \vec{S}_2 \cdot \vec{v}_1 \vec{v}_1 \cdot \vec{v}_2 + 6 \vec{S}_1 \cdot \vec{S}_2 \vec{v}_1 \cdot \vec{v}_1 \vec{v}_1 \cdot \vec{v}_2 \Big) m_1 \Big\}
 \end{aligned}$$

{DiagS1S2[2, 2, 16],

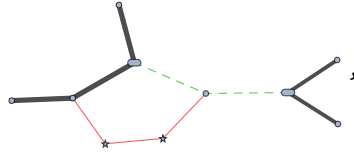

$$\begin{aligned}
 G^2 \left( \frac{1}{r} \left( -\frac{4}{3} \hat{n} \cdot \vec{S}_1 \hat{n} \cdot \vec{S}_2 \hat{n} \cdot \vec{a}_1 - \frac{2}{3} \hat{n} \cdot \vec{S}_2 \hat{n} \cdot \vec{S}_1 \hat{n} \cdot \vec{a}_1 - \frac{2}{3} \hat{n} \cdot \vec{S}_1 \hat{n} \cdot \vec{S}_2 \hat{n} \cdot \vec{a}_1 + \frac{1}{6} \vec{S}_1 \cdot \vec{S}_2 \hat{n} \cdot \vec{a}_1 + \frac{1}{12} \vec{S}_1 \cdot \vec{S}_2 \hat{n} \cdot \vec{a}_1 + \frac{1}{12} \vec{S}_1 \cdot \vec{S}_2 \right. \right. \\
 \hat{n} \cdot \vec{a}_1 + \frac{2}{3} \hat{n} \cdot \vec{S}_2 \vec{S}_1 \cdot \vec{a}_1 + \frac{1}{3} \hat{n} \cdot \vec{S}_2 \vec{S}_1 \cdot \vec{a}_1 - \frac{5}{6} \hat{n} \cdot \vec{S}_1 \vec{S}_2 \cdot \vec{a}_1 - \frac{5}{12} \hat{n} \cdot \vec{S}_1 \vec{S}_2 \cdot \vec{a}_1 + \frac{1}{3} \hat{n} \cdot \vec{S}_2 \vec{S}_1 \cdot \vec{a}_1 - \frac{5}{12} \hat{n} \cdot \vec{S}_1 \vec{S}_2 \cdot \vec{a}_1 \Big) + \\
 \frac{1}{r^2} \left( \frac{7}{2} \hat{n} \cdot \vec{S}_1 \hat{n} \cdot \vec{S}_2 (\hat{n} \cdot \vec{a}_1)^2 + \frac{1}{4} \vec{S}_1 \cdot \vec{S}_2 (\hat{n} \cdot \vec{a}_1)^2 - \frac{8}{3} \hat{n} \cdot \vec{a}_2 \hat{n} \cdot \vec{S}_1 \hat{n} \cdot \vec{S}_2 \hat{n} \cdot \vec{a}_1 + 7 \hat{n} \cdot \vec{S}_2 \hat{n} \cdot \vec{S}_1 \hat{n} \cdot \vec{v}_1 \hat{n} \cdot \vec{a}_1 + \right. \\
 7 \hat{n} \cdot \vec{S}_1 \hat{n} \cdot \vec{S}_2 \hat{n} \cdot \vec{v}_1 \hat{n} \cdot \vec{a}_1 - \frac{16}{3} \hat{n} \cdot \vec{S}_2 \hat{n} \cdot \vec{S}_1 \hat{n} \cdot \vec{v}_2 \hat{n} \cdot \vec{a}_1 - \frac{16}{3} \hat{n} \cdot \vec{S}_1 \hat{n} \cdot \vec{S}_2 \hat{n} \cdot \vec{v}_2 \hat{n} \cdot \vec{a}_1 + \frac{1}{2} \hat{n} \cdot \vec{v}_1 \vec{S}_1 \cdot \vec{S}_2 \hat{n} \cdot \vec{a}_1 + \\
 \frac{1}{3} \hat{n} \cdot \vec{v}_2 \vec{S}_1 \cdot \vec{S}_2 \hat{n} \cdot \vec{a}_1 - \frac{7}{4} \hat{n} \cdot \vec{S}_2 \vec{S}_1 \cdot \vec{v}_1 \hat{n} \cdot \vec{a}_1 + \frac{4}{3} \hat{n} \cdot \vec{S}_2 \vec{S}_1 \cdot \vec{v}_2 \hat{n} \cdot \vec{a}_1 - \frac{7}{4} \hat{n} \cdot \vec{S}_1 \vec{S}_2 \cdot \vec{v}_1 \hat{n} \cdot \vec{a}_1 + \frac{4}{3} \hat{n} \cdot \vec{S}_1 \vec{S}_2 \cdot \vec{v}_2 \hat{n} \cdot \vec{a}_1 + \\
 \frac{1}{2} \hat{n} \cdot \vec{v}_1 \vec{S}_1 \cdot \vec{S}_2 \hat{n} \cdot \vec{a}_1 + \frac{1}{3} \hat{n} \cdot \vec{v}_2 \vec{S}_1 \cdot \vec{S}_2 \hat{n} \cdot \vec{a}_1 - \frac{7}{4} \hat{n} \cdot \vec{S}_2 \vec{S}_1 \cdot \vec{a}_1 \hat{n} \cdot \vec{a}_1 + \frac{2}{3} \hat{n} \cdot \vec{S}_2 \vec{S}_1 \cdot \vec{a}_2 \hat{n} \cdot \vec{a}_1 + \\
 \frac{1}{6} \hat{n} \cdot \vec{a}_2 \vec{S}_1 \cdot \vec{S}_2 \hat{n} \cdot \vec{a}_1 - \frac{7}{4} \hat{n} \cdot \vec{S}_2 \vec{S}_1 \cdot \vec{v}_1 \hat{n} \cdot \vec{a}_1 + \frac{4}{3} \hat{n} \cdot \vec{S}_2 \vec{S}_1 \cdot \vec{v}_2 \hat{n} \cdot \vec{a}_1 - \frac{1}{4} \hat{n} \cdot \vec{S}_1 \vec{S}_2 \cdot \vec{a}_1 \hat{n} \cdot \vec{a}_1 + \\
 \frac{2}{3} \hat{n} \cdot \vec{S}_1 \vec{S}_2 \cdot \vec{a}_2 \hat{n} \cdot \vec{a}_1 - \frac{7}{4} \hat{n} \cdot \vec{S}_1 \vec{S}_2 \cdot \vec{v}_1 \hat{n} \cdot \vec{a}_1 + \frac{4}{3} \hat{n} \cdot \vec{S}_1 \vec{S}_2 \cdot \vec{v}_2 \hat{n} \cdot \vec{a}_1 - \frac{5}{3} \hat{n} \cdot \vec{S}_1 \hat{n} \cdot \vec{S}_2 (\hat{n} \cdot \vec{v}_1)^2 - \Big)
 \end{aligned}$$



[illegible]

[illegible]

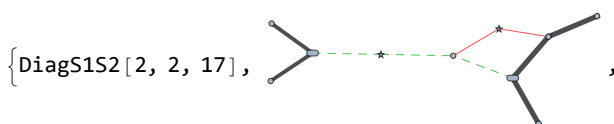

$$G^2 \left( \frac{1}{r} \left( \frac{1}{3} \hat{n} \cdot \vec{S}_1 \hat{n} \cdot \vec{S}_2 \hat{n} \cdot \vec{a}_1 + \frac{1}{3} \hat{n} \cdot \vec{S}_2 \hat{n} \cdot \vec{S}_1 \hat{n} \cdot \vec{a}_1 - \frac{5}{12} \vec{S}_1 \cdot \vec{S}_2 \hat{n} \cdot \vec{a}_1 - \frac{5}{12} \vec{S}_1 \cdot \vec{S}_2 \hat{n} \cdot \vec{a}_1 + \frac{1}{3} \hat{n} \cdot \vec{S}_1 \hat{n} \cdot \vec{S}_2 \hat{n} \cdot \vec{v}_1 + \right. \right. \\ \left. \left. \frac{1}{3} \hat{n} \cdot \vec{S}_1 \hat{n} \cdot \vec{S}_2 \hat{n} \cdot \vec{v}_1 - \frac{5}{12} \hat{n} \cdot \vec{v}_1 \vec{S}_1 \cdot \vec{S}_2 - \frac{1}{6} \hat{n} \cdot \vec{S}_2 \vec{S}_1 \cdot \vec{a}_1 - \frac{1}{6} \hat{n} \cdot \vec{S}_2 \vec{S}_1 \cdot \vec{v}_1 - \frac{5}{12} \hat{n} \cdot \vec{v}_1 \vec{S}_1 \cdot \vec{S}_2 - \right. \right.$$











$\{\text{DiagS1S2}[2, 2, 19],$

,

[illegible]



[illegible]

$$\begin{aligned}
& 12 \hat{n} \times \vec{S}_1 \cdot \vec{v}_1 \hat{n} \times \vec{S}_2 \cdot \vec{v}_1 (\hat{n} \cdot \vec{v}_2)^2 - \frac{5}{2} \hat{n} \cdot \vec{S}_1 \hat{n} \cdot \vec{S}_2 (\vec{v}_1 \cdot \vec{v}_1)^2 + \frac{3}{4} \vec{S}_1 \cdot \vec{S}_2 (\vec{v}_1 \cdot \vec{v}_1)^2 - 6 \hat{n} \cdot \vec{S}_1 \hat{n} \cdot \vec{S}_2 (\vec{v}_1 \cdot \vec{v}_2)^2 - \\
& \vec{S}_1 \cdot \vec{S}_2 (\vec{v}_1 \cdot \vec{v}_2)^2 + \vec{S}_1 \times \vec{v}_1 \cdot \vec{v}_2 \vec{S}_2 \times \vec{v}_1 \cdot \vec{v}_2 - 4 \hat{n} \times \vec{S}_2 \cdot \vec{v}_1 \vec{S}_1 \times \vec{v}_1 \cdot \vec{v}_2 \hat{n} \cdot \vec{v}_2 - 4 \hat{n} \times \vec{S}_1 \cdot \vec{v}_1 \vec{S}_2 \times \vec{v}_1 \cdot \vec{v}_2 \hat{n} \cdot \vec{v}_2 - \\
& 12 \hat{n} \cdot \vec{S}_1 \hat{n} \cdot \vec{S}_2 (\hat{n} \cdot \vec{v}_2)^2 \vec{v}_1 \cdot \vec{v}_1 - \frac{5}{2} \hat{n} \times \vec{S}_1 \cdot \vec{v}_1 \hat{n} \times \vec{S}_2 \cdot \vec{v}_1 \vec{v}_1 \cdot \vec{v}_1 + 4 \hat{n} \cdot \vec{S}_2 \hat{n} \cdot \vec{v}_2 \vec{S}_1 \cdot \vec{v}_1 \vec{v}_1 \cdot \vec{v}_1 + \\
& 4 \hat{n} \cdot \vec{S}_2 \hat{n} \cdot \vec{v}_2 \vec{S}_1 \cdot \vec{v}_2 \vec{v}_1 \cdot \vec{v}_1 + \frac{1}{2} \vec{S}_1 \cdot \vec{v}_1 \vec{S}_2 \cdot \vec{v}_1 \vec{v}_1 \cdot \vec{v}_1 + 4 \hat{n} \cdot \vec{S}_1 \hat{n} \cdot \vec{v}_2 \vec{S}_2 \cdot \vec{v}_2 \vec{v}_1 \cdot \vec{v}_1 - \vec{S}_1 \cdot \vec{v}_1 \vec{S}_2 \cdot \vec{v}_2 \vec{v}_1 \cdot \vec{v}_1 - \\
& \vec{S}_1 \cdot \vec{v}_2 \vec{S}_2 \cdot \vec{v}_2 \vec{v}_1 \cdot \vec{v}_1 + 2 \hat{n} \times \vec{S}_1 \cdot \vec{v}_1 \hat{n} \times \vec{S}_2 \cdot \vec{v}_1 \vec{v}_1 \cdot \vec{v}_2 - 12 \hat{n} \cdot \vec{S}_2 \hat{n} \cdot \vec{v}_2 \vec{S}_1 \cdot \vec{v}_1 \vec{v}_1 \cdot \vec{v}_2 - 4 \hat{n} \cdot \vec{S}_1 \hat{n} \cdot \vec{v}_2 \vec{S}_2 \cdot \vec{v}_1 \vec{v}_1 \cdot \vec{v}_2 - \\
& 2 \vec{S}_1 \cdot \vec{v}_1 \vec{S}_2 \cdot \vec{v}_1 \vec{v}_1 \cdot \vec{v}_2 + \vec{S}_1 \cdot \vec{v}_2 \vec{S}_2 \cdot \vec{v}_1 \vec{v}_1 \cdot \vec{v}_2 + 3 \vec{S}_1 \cdot \vec{v}_1 \vec{S}_2 \cdot \vec{v}_2 \vec{v}_1 \cdot \vec{v}_2 + 4 \hat{n} \cdot \vec{S}_1 \hat{n} \cdot \vec{S}_2 \vec{v}_1 \cdot \vec{v}_1 \vec{v}_1 \cdot \vec{v}_2 + \\
& \vec{S}_1 \cdot \vec{S}_2 \vec{v}_1 \cdot \vec{v}_1 \vec{v}_1 \cdot \vec{v}_2 - 2 \hat{n} \times \vec{S}_1 \cdot \vec{v}_1 \hat{n} \times \vec{S}_2 \cdot \vec{v}_1 \vec{v}_2 \cdot \vec{v}_2 + 2 \hat{n} \cdot \vec{S}_1 \hat{n} \cdot \vec{S}_2 \vec{v}_1 \cdot \vec{v}_1 \vec{v}_2 \cdot \vec{v}_2 \Big) \Big) m_1 \Big\}
\end{aligned}$$

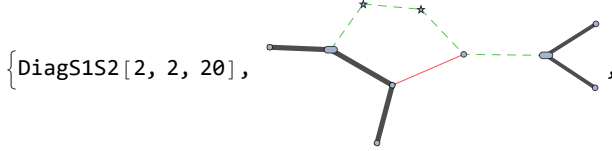

$$\begin{aligned}
G^2 m_1 \Big( & -\frac{1}{6} \hat{n} \cdot \vec{S}_1 \hat{n} \cdot \vec{S}_2 + \frac{17}{18} \vec{S}_1 \cdot \vec{S}_2 + \frac{1}{r} \left( \hat{n} \cdot \vec{S}_2 \hat{n} \cdot \vec{a}_1 \hat{n} \cdot \vec{S}_1 - \frac{3}{4} \vec{S}_2 \cdot \vec{a}_1 \hat{n} \cdot \vec{S}_1 - \frac{2}{3} \hat{n} \cdot \vec{S}_1 \hat{n} \cdot \vec{a}_1 \hat{n} \cdot \vec{S}_2 - \right. \\
& \frac{1}{3} \hat{n} \cdot \vec{S}_1 \hat{n} \cdot \vec{a}_2 \hat{n} \cdot \vec{S}_2 - \frac{4}{3} \hat{n} \cdot \vec{S}_1 \hat{n} \cdot \vec{S}_2 \hat{n} \cdot \vec{v}_1 + 2 \hat{n} \cdot \vec{S}_1 \hat{n} \cdot \vec{S}_2 \hat{n} \cdot \vec{v}_1 - \frac{2}{3} \hat{n} \cdot \vec{S}_1 \hat{n} \cdot \vec{S}_2 \hat{n} \cdot \vec{v}_2 + \\
& \frac{5}{2} \hat{n} \cdot \vec{v}_1 \vec{S}_1 \cdot \vec{S}_2 - \hat{n} \cdot \vec{S}_2 \vec{S}_1 \cdot \vec{v}_1 - \frac{11}{6} \hat{n} \cdot \vec{v}_1 \vec{S}_1 \cdot \vec{S}_2 - \frac{2}{3} \hat{n} \cdot \vec{v}_2 \vec{S}_1 \cdot \vec{S}_2 + \frac{1}{3} \hat{n} \cdot \vec{S}_2 \vec{S}_1 \cdot \vec{a}_1 + \frac{1}{6} \hat{n} \cdot \vec{S}_2 \vec{S}_1 \cdot \vec{a}_2 - \\
& \frac{11}{12} \hat{n} \cdot \vec{a}_1 \vec{S}_1 \cdot \vec{S}_2 - \frac{1}{3} \hat{n} \cdot \vec{a}_2 \vec{S}_1 \cdot \vec{S}_2 + \frac{2}{3} \hat{n} \cdot \vec{S}_2 \vec{S}_1 \cdot \vec{v}_1 + \frac{1}{3} \hat{n} \cdot \vec{S}_2 \vec{S}_1 \cdot \vec{v}_2 + \frac{7}{6} \hat{n} \cdot \vec{S}_1 \vec{S}_2 \cdot \vec{v}_1 + \frac{1}{3} \hat{n} \cdot \vec{S}_1 \vec{S}_2 \cdot \vec{v}_2 - \\
& \frac{3}{2} \hat{n} \cdot \vec{S}_1 \vec{S}_2 \cdot \vec{v}_1 + \frac{5}{4} \hat{n} \cdot \vec{a}_1 \vec{S}_1 \cdot \vec{S}_2 - \frac{1}{2} \hat{n} \cdot \vec{S}_2 \vec{S}_1 \cdot \vec{a}_1 + \frac{7}{12} \hat{n} \cdot \vec{S}_1 \vec{S}_2 \cdot \vec{a}_1 + \frac{1}{6} \hat{n} \cdot \vec{S}_1 \vec{S}_2 \cdot \vec{a}_2 \Big) + \frac{1}{r^2} \\
& \left( -\frac{11}{6} \hat{n} \cdot \vec{S}_1 \hat{n} \cdot \vec{S}_2 (\hat{n} \cdot \vec{a}_1)^2 - \frac{5}{12} \vec{S}_1 \cdot \vec{S}_2 (\hat{n} \cdot \vec{a}_1)^2 + 4 \hat{n} \cdot \vec{a}_2 \hat{n} \cdot \vec{S}_1 \hat{n} \cdot \vec{S}_2 \hat{n} \cdot \vec{a}_1 - \frac{11}{3} \hat{n} \cdot \vec{S}_2 \hat{n} \cdot \vec{S}_1 \hat{n} \cdot \vec{v}_1 \hat{n} \cdot \vec{a}_1 - \right. \\
& \frac{11}{3} \hat{n} \cdot \vec{S}_1 \hat{n} \cdot \vec{S}_2 \hat{n} \cdot \vec{v}_1 \hat{n} \cdot \vec{a}_1 + 8 \hat{n} \cdot \vec{S}_2 \hat{n} \cdot \vec{S}_1 \hat{n} \cdot \vec{v}_2 \hat{n} \cdot \vec{a}_1 - \frac{5}{6} \hat{n} \cdot \vec{v}_1 \vec{S}_1 \cdot \vec{S}_2 \hat{n} \cdot \vec{a}_1 + \frac{11}{12} \hat{n} \cdot \vec{S}_2 \vec{S}_1 \cdot \vec{v}_1 \hat{n} \cdot \vec{a}_1 - \\
& \frac{1}{12} \hat{n} \cdot \vec{S}_1 \vec{S}_2 \cdot \vec{v}_1 \hat{n} \cdot \vec{a}_1 - 2 \hat{n} \cdot \vec{S}_1 \vec{S}_2 \cdot \vec{v}_2 \hat{n} \cdot \vec{a}_1 - \frac{5}{6} \hat{n} \cdot \vec{v}_1 \vec{S}_1 \cdot \vec{S}_2 \hat{n} \cdot \vec{a}_1 + 5 \hat{n} \cdot \vec{v}_2 \vec{S}_1 \cdot \vec{S}_2 \hat{n} \cdot \vec{a}_1 + \\
& \frac{11}{12} \hat{n} \cdot \vec{S}_2 \vec{S}_1 \cdot \vec{a}_1 \hat{n} \cdot \vec{a}_1 - \hat{n} \cdot \vec{S}_2 \vec{S}_1 \cdot \vec{a}_2 \hat{n} \cdot \vec{a}_1 + \frac{5}{2} \hat{n} \cdot \vec{a}_2 \vec{S}_1 \cdot \vec{S}_2 \hat{n} \cdot \vec{a}_1 + \frac{11}{12} \hat{n} \cdot \vec{S}_2 \vec{S}_1 \cdot \vec{v}_1 \hat{n} \cdot \vec{a}_1 - 2 \hat{n} \cdot \vec{S}_2 \vec{S}_1 \cdot \vec{v}_2 \hat{n} \cdot \vec{a}_1 + \\
& \frac{5}{12} \hat{n} \cdot \vec{S}_1 \vec{S}_2 \cdot \vec{a}_1 \hat{n} \cdot \vec{a}_1 - \hat{n} \cdot \vec{S}_1 \vec{S}_2 \cdot \vec{a}_2 \hat{n} \cdot \vec{a}_1 + \frac{11}{12} \hat{n} \cdot \vec{S}_1 \vec{S}_2 \cdot \vec{v}_1 \hat{n} \cdot \vec{a}_1 - \frac{22}{3} \hat{n} \cdot \vec{S}_1 \hat{n} \cdot \vec{S}_2 (\hat{n} \cdot \vec{v}_1)^2 - \\
& \frac{13}{6} \hat{n} \cdot \vec{S}_2 \hat{n} \cdot \vec{S}_1 (\hat{n} \cdot \vec{v}_1)^2 + \frac{9}{2} \hat{n} \cdot \vec{S}_1 \hat{n} \cdot \vec{S}_2 (\hat{n} \cdot \vec{v}_1)^2 - \frac{4}{3} \hat{n} \cdot \vec{S}_1 \hat{n} \cdot \vec{S}_2 (\hat{n} \cdot \vec{v}_2)^2 + 3 \hat{n} \times \vec{S}_1 \cdot \vec{v}_1 \hat{n} \times \vec{S}_2 \cdot \vec{v}_1 + \\
& \frac{3}{4} \hat{n} \times \vec{S}_2 \cdot \vec{v}_1 \hat{n} \times \vec{S}_1 \cdot \vec{a}_1 + \frac{3}{4} \hat{n} \times \vec{S}_2 \cdot \vec{a}_1 \hat{n} \times \vec{S}_1 \cdot \vec{v}_1 - \frac{3}{4} \hat{n} \times \vec{S}_2 \cdot \vec{v}_1 \hat{n} \times \vec{S}_1 \cdot \vec{v}_1 + \frac{3}{4} \hat{n} \times \vec{S}_1 \cdot \vec{v}_1 \hat{n} \times \vec{S}_2 \cdot \vec{a}_1 + \\
& \frac{3}{4} \hat{n} \times \vec{S}_1 \cdot \vec{a}_1 \hat{n} \times \vec{S}_2 \cdot \vec{a}_1 + \frac{3}{4} \hat{n} \times \vec{S}_1 \cdot \vec{a}_1 \hat{n} \times \vec{S}_2 \cdot \vec{v}_1 - \frac{3}{4} \hat{n} \times \vec{S}_1 \cdot \vec{v}_1 \hat{n} \times \vec{S}_2 \cdot \vec{v}_1 + 8 \hat{n} \cdot \vec{S}_1 \hat{n} \cdot \vec{a}_2 \hat{n} \cdot \vec{S}_2 \hat{n} \cdot \vec{v}_1 + \\
& 16 \hat{n} \cdot \vec{S}_1 \hat{n} \cdot \vec{S}_2 \hat{n} \cdot \vec{v}_1 \hat{n} \cdot \vec{v}_2 - \frac{16}{3} \hat{n} \cdot \vec{S}_1 \hat{n} \cdot \vec{S}_2 \hat{n} \cdot \vec{v}_1 \hat{n} \cdot \vec{v}_2 - \frac{5}{3} (\hat{n} \cdot \vec{v}_1)^2 \vec{S}_1 \cdot \vec{S}_2 + 10 \hat{n} \cdot \vec{v}_1 \hat{n} \cdot \vec{v}_2 \vec{S}_1 \cdot \vec{S}_2 + \\
& \frac{11}{12} \hat{n} \cdot \vec{S}_2 \hat{n} \cdot \vec{v}_1 \vec{S}_1 \cdot \vec{a}_1 - 2 \hat{n} \cdot \vec{S}_2 \hat{n} \cdot \vec{v}_1 \vec{S}_1 \cdot \vec{a}_2 + 5 \hat{n} \cdot \vec{a}_2 \hat{n} \cdot \vec{v}_1 \vec{S}_1 \cdot \vec{S}_2 - 2 \hat{n} \cdot \vec{a}_2 \hat{n} \cdot \vec{S}_2 \vec{S}_1 \cdot \vec{v}_1 + \\
& \frac{11}{3} \hat{n} \cdot \vec{S}_2 \hat{n} \cdot \vec{v}_1 \vec{S}_1 \cdot \vec{v}_1 - 4 \hat{n} \cdot \vec{S}_2 \hat{n} \cdot \vec{v}_2 \vec{S}_1 \cdot \vec{v}_1 - 4 \hat{n} \cdot \vec{S}_2 \hat{n} \cdot \vec{v}_1 \vec{S}_1 \cdot \vec{v}_2 + \frac{9}{4} (\hat{n} \cdot \vec{v}_1)^2 \vec{S}_1 \cdot \vec{S}_2 - \frac{2}{3} (\hat{n} \cdot \vec{v}_2)^2 \vec{S}_1 \cdot \vec{S}_2 - \\
& \frac{11}{3} \hat{n} \cdot \vec{v}_1 \hat{n} \cdot \vec{v}_2 \vec{S}_1 \cdot \vec{S}_2 - \frac{9}{4} \hat{n} \cdot \vec{S}_2 \hat{n} \cdot \vec{v}_1 \vec{S}_1 \cdot \vec{v}_1 + \frac{4}{3} \hat{n} \cdot \vec{S}_2 \hat{n} \cdot \vec{v}_2 \vec{S}_1 \cdot \vec{v}_1 + \frac{4}{3} \hat{n} \cdot \vec{S}_2 \hat{n} \cdot \vec{v}_1 \vec{S}_1 \cdot \vec{v}_2 +
\end{aligned}$$









$$\left. \frac{17}{3} \hat{n} \cdot \vec{S}_1 \hat{n} \cdot \vec{S}_2 \vec{v}_1 \cdot \vec{v}_1 \vec{v}_2 \cdot \vec{v}_2 - \frac{17}{6} \vec{S}_1 \cdot \vec{S}_2 \vec{v}_1 \cdot \vec{v}_1 \vec{v}_2 \cdot \vec{v}_2 \right) + \frac{1}{3} \vec{S}_1 \cdot \vec{S}_2 \log\left(\frac{r}{R_\theta}\right) - \frac{\vec{S}_1 \cdot \vec{S}_2}{6 \epsilon_d} \Bigg\}$$

{DiagS1S2[2, 2, 21], 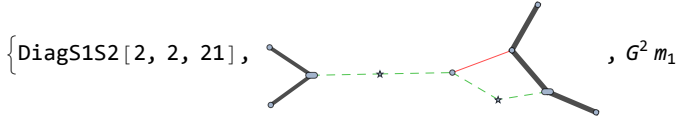,  $G^2 m_1$

$$\begin{aligned} & \left( - \left( \hat{n} \cdot \vec{S}_1 \right) \hat{n} \cdot \vec{S}_2 + \frac{1}{r} \left( \hat{n} \cdot \vec{S}_1 \hat{n} \cdot \vec{S}_2 \hat{n} \cdot \vec{a}_1 + \hat{n} \cdot \vec{S}_2 \hat{n} \cdot \vec{S}_1 \hat{n} \cdot \vec{a}_1 + \frac{3}{4} \vec{S}_1 \cdot \vec{S}_2 \hat{n} \cdot \vec{a}_1 + \frac{5}{4} \vec{S}_1 \cdot \vec{S}_2 \hat{n} \cdot \vec{a}_1 - 2 \hat{n} \cdot \vec{S}_1 \hat{n} \cdot \vec{a}_2 \hat{n} \cdot \vec{S}_2 + \right. \right. \\ & \quad \hat{n} \cdot \vec{S}_1 \hat{n} \cdot \vec{S}_2 \hat{n} \cdot \vec{v}_1 + 3 \hat{n} \cdot \vec{S}_1 \hat{n} \cdot \vec{S}_2 \hat{n} \cdot \vec{v}_1 - 4 \hat{n} \cdot \vec{S}_1 \hat{n} \cdot \vec{S}_2 \hat{n} \cdot \vec{v}_2 + \frac{13}{4} \hat{n} \cdot \vec{v}_1 \vec{S}_1 \cdot \vec{S}_2 - \frac{1}{2} \hat{n} \cdot \vec{S}_2 \vec{S}_1 \cdot \vec{a}_1 - \frac{3}{2} \hat{n} \cdot \vec{S}_2 \vec{S}_1 \cdot \vec{v}_1 + \\ & \quad \frac{3}{4} \hat{n} \cdot \vec{v}_1 \vec{S}_1 \cdot \vec{S}_2 - 4 \hat{n} \cdot \vec{v}_2 \vec{S}_1 \cdot \vec{S}_2 + \hat{n} \cdot \vec{S}_2 \vec{S}_1 \cdot \vec{a}_2 - 2 \hat{n} \cdot \vec{a}_2 \vec{S}_1 \cdot \vec{S}_2 - \frac{1}{2} \hat{n} \cdot \vec{S}_2 \vec{S}_1 \cdot \vec{v}_1 + 2 \hat{n} \cdot \vec{S}_2 \vec{S}_1 \cdot \vec{v}_2 - \frac{1}{4} \hat{n} \cdot \vec{S}_1 \vec{S}_2 \cdot \vec{a}_1 - \\ & \quad \left. \frac{1}{4} \hat{n} \cdot \vec{S}_1 \vec{S}_2 \cdot \vec{v}_1 + 2 \hat{n} \cdot \vec{S}_1 \vec{S}_2 \cdot \vec{v}_2 - \frac{3}{4} \hat{n} \cdot \vec{S}_1 \vec{S}_2 \cdot \vec{a}_1 - \frac{7}{4} \hat{n} \cdot \vec{S}_1 \vec{S}_2 \cdot \vec{v}_1 - \frac{1}{2} \hat{n} \cdot \vec{S}_2 \vec{S}_1 \cdot \vec{a}_1 + \hat{n} \cdot \vec{S}_1 \vec{S}_2 \cdot \vec{a}_2 \right) + \\ & \quad \frac{1}{r^2} \left( -5 \hat{n} \cdot \vec{S}_1 \hat{n} \cdot \vec{S}_2 (\hat{n} \cdot \vec{v}_1)^2 - 4 \hat{n} \cdot \vec{S}_2 \hat{n} \cdot \vec{S}_1 (\hat{n} \cdot \vec{v}_1)^2 - \frac{5}{2} \vec{S}_1 \cdot \vec{S}_2 (\hat{n} \cdot \vec{v}_1)^2 - \frac{5}{2} \vec{S}_1 \cdot \vec{S}_2 (\hat{n} \cdot \vec{v}_1)^2 - \right. \\ & \quad 2 \hat{n} \cdot \vec{S}_2 \hat{n} \cdot \vec{a}_1 \hat{n} \cdot \vec{S}_1 \hat{n} \cdot \vec{v}_1 + 12 \hat{n} \cdot \vec{S}_1 \hat{n} \cdot \vec{a}_2 \hat{n} \cdot \vec{S}_2 \hat{n} \cdot \vec{v}_1 + 24 \hat{n} \cdot \vec{S}_1 \hat{n} \cdot \vec{S}_2 \hat{n} \cdot \vec{v}_2 \hat{n} \cdot \vec{v}_1 + 4 \hat{n} \cdot \vec{S}_1 \hat{n} \cdot \vec{S}_2 \hat{n} \cdot \vec{v}_2 \hat{n} \cdot \vec{v}_1 + \\ & \quad 13 \hat{n} \cdot \vec{v}_2 \vec{S}_1 \cdot \vec{S}_2 \hat{n} \cdot \vec{v}_1 - 3 \hat{n} \cdot \vec{S}_2 \vec{S}_1 \cdot \vec{a}_2 \hat{n} \cdot \vec{v}_1 + \frac{13}{2} \hat{n} \cdot \vec{a}_2 \vec{S}_1 \cdot \vec{S}_2 \hat{n} \cdot \vec{v}_1 + \frac{5}{2} \hat{n} \cdot \vec{S}_2 \vec{S}_1 \cdot \vec{v}_1 \hat{n} \cdot \vec{v}_1 - \\ & \quad 6 \hat{n} \cdot \vec{S}_2 \vec{S}_1 \cdot \vec{v}_2 \hat{n} \cdot \vec{v}_1 + \frac{3}{2} \hat{n} \cdot \vec{v}_2 \vec{S}_1 \cdot \vec{S}_2 \hat{n} \cdot \vec{v}_1 - \hat{n} \cdot \vec{S}_2 \vec{S}_1 \cdot \vec{v}_2 \hat{n} \cdot \vec{v}_1 + \hat{n} \cdot \vec{S}_1 \vec{S}_2 \cdot \vec{a}_1 \hat{n} \cdot \vec{v}_1 + \frac{5}{2} \hat{n} \cdot \vec{S}_1 \vec{S}_2 \cdot \vec{v}_1 \hat{n} \cdot \vec{v}_1 - \\ & \quad 6 \hat{n} \cdot \vec{S}_1 \vec{S}_2 \cdot \vec{v}_2 \hat{n} \cdot \vec{v}_1 + \frac{5}{2} \hat{n} \cdot \vec{S}_1 \vec{S}_2 \cdot \vec{v}_1 \hat{n} \cdot \vec{v}_1 - 2 \hat{n} \cdot \vec{a}_1 \vec{S}_1 \cdot \vec{S}_2 \hat{n} \cdot \vec{v}_1 + \frac{1}{2} \hat{n} \cdot \vec{S}_2 \vec{S}_1 \cdot \vec{a}_1 \hat{n} \cdot \vec{v}_1 + 2 \hat{n} \cdot \vec{S}_2 \vec{S}_1 \cdot \vec{v}_1 \hat{n} \cdot \vec{v}_1 - \\ & \quad 3 \hat{n} \cdot \vec{S}_1 \vec{S}_2 \cdot \vec{a}_2 \hat{n} \cdot \vec{v}_1 - \hat{n} \cdot \vec{S}_1 \vec{S}_2 \cdot \vec{v}_2 \hat{n} \cdot \vec{v}_1 - 8 \hat{n} \cdot \vec{S}_1 \hat{n} \cdot \vec{S}_2 (\hat{n} \cdot \vec{v}_2)^2 - \frac{1}{2} \hat{n} \times \vec{S}_1 \cdot \vec{v}_1 \hat{n} \times \vec{S}_2 \cdot \vec{v}_1 - \\ & \quad \frac{1}{2} \hat{n} \times \vec{S}_2 \cdot \vec{v}_1 \hat{n} \times \vec{S}_1 \cdot \vec{a}_1 - \frac{1}{2} \hat{n} \times \vec{S}_2 \cdot \vec{a}_1 \hat{n} \times \vec{S}_1 \cdot \vec{v}_1 + 4 \hat{n} \cdot \vec{a}_1 \hat{n} \cdot \vec{a}_2 \hat{n} \cdot \vec{S}_1 \hat{n} \cdot \vec{S}_2 + 8 \hat{n} \cdot \vec{S}_2 \hat{n} \cdot \vec{a}_1 \hat{n} \cdot \vec{S}_1 \hat{n} \cdot \vec{v}_2 + \\ & \quad 4 \hat{n} \cdot \vec{S}_1 \hat{n} \cdot \vec{a}_1 \hat{n} \cdot \vec{S}_2 \hat{n} \cdot \vec{v}_2 - \hat{n} \cdot \vec{S}_2 \hat{n} \cdot \vec{v}_2 \vec{S}_1 \cdot \vec{a}_1 + \frac{3}{2} \hat{n} \cdot \vec{a}_1 \hat{n} \cdot \vec{v}_2 \vec{S}_1 \cdot \vec{S}_2 - 3 \hat{n} \cdot \vec{a}_2 \hat{n} \cdot \vec{S}_2 \vec{S}_1 \cdot \vec{v}_1 - \\ & \quad 6 \hat{n} \cdot \vec{S}_2 \hat{n} \cdot \vec{v}_2 \vec{S}_1 \cdot \vec{v}_1 - \hat{n} \cdot \vec{a}_1 \hat{n} \cdot \vec{S}_2 \vec{S}_1 \cdot \vec{v}_2 - 4 (\hat{n} \cdot \vec{v}_2)^2 \vec{S}_1 \cdot \vec{S}_2 - \hat{n} \cdot \vec{S}_2 \hat{n} \cdot \vec{v}_2 \vec{S}_1 \cdot \vec{v}_1 + 4 \hat{n} \cdot \vec{S}_2 \hat{n} \cdot \vec{v}_2 \vec{S}_1 \cdot \vec{v}_2 - \\ & \quad 3 \hat{n} \cdot \vec{S}_1 \hat{n} \cdot \vec{v}_2 \vec{S}_2 \cdot \vec{a}_1 + \hat{n} \cdot \vec{a}_1 \hat{n} \cdot \vec{S}_1 \vec{S}_2 \cdot \vec{v}_1 - 7 \hat{n} \cdot \vec{S}_1 \hat{n} \cdot \vec{v}_2 \vec{S}_2 \cdot \vec{v}_1 - \frac{3}{2} \vec{S}_1 \cdot \vec{v}_1 \vec{S}_2 \cdot \vec{v}_1 + \frac{7}{2} \vec{S}_1 \cdot \vec{v}_2 \vec{S}_2 \cdot \vec{v}_1 - \\ & \quad 2 \hat{n} \cdot \vec{a}_1 \hat{n} \cdot \vec{S}_1 \vec{S}_2 \cdot \vec{v}_2 + 3 \vec{S}_1 \cdot \vec{v}_1 \vec{S}_2 \cdot \vec{v}_2 - \hat{n} \cdot \vec{S}_1 \hat{n} \cdot \vec{S}_2 \vec{a}_1 \cdot \vec{a}_2 - 2 \hat{n} \cdot \vec{S}_2 \hat{n} \cdot \vec{S}_1 \vec{a}_1 \cdot \vec{v}_2 - \hat{n} \cdot \vec{S}_1 \hat{n} \cdot \vec{S}_2 \vec{a}_1 \cdot \vec{v}_2 - \\ & \quad \frac{3}{4} \vec{S}_1 \cdot \vec{S}_2 \vec{a}_1 \cdot \vec{v}_2 + 5 \hat{n} \cdot \vec{a}_1 \hat{n} \cdot \vec{v}_2 \vec{S}_1 \cdot \vec{S}_2 - \frac{5}{2} \vec{a}_1 \cdot \vec{v}_2 \vec{S}_1 \cdot \vec{S}_2 - \hat{n} \cdot \vec{a}_2 \hat{n} \cdot \vec{S}_2 \vec{S}_1 \cdot \vec{a}_1 - 2 \hat{n} \cdot \vec{S}_2 \hat{n} \cdot \vec{v}_2 \vec{S}_1 \cdot \vec{a}_1 - \\ & \quad \frac{3}{4} \vec{S}_2 \cdot \vec{v}_1 \vec{S}_1 \cdot \vec{a}_1 + \vec{S}_2 \cdot \vec{v}_2 \vec{S}_1 \cdot \vec{a}_1 - \hat{n} \cdot \vec{a}_1 \hat{n} \cdot \vec{S}_2 \vec{S}_1 \cdot \vec{a}_2 + \frac{5}{2} \hat{n} \cdot \vec{a}_1 \hat{n} \cdot \vec{a}_2 \vec{S}_1 \cdot \vec{S}_2 - \frac{5}{4} \vec{a}_1 \cdot \vec{a}_2 \vec{S}_1 \cdot \vec{S}_2 + \\ & \quad \frac{1}{2} \hat{n} \cdot \vec{S}_2 \hat{n} \cdot \vec{a}_1 \vec{S}_1 \cdot \vec{v}_1 - \frac{3}{4} \vec{S}_2 \cdot \vec{a}_1 \vec{S}_1 \cdot \vec{v}_1 - \frac{5}{4} \vec{S}_2 \cdot \vec{v}_1 \vec{S}_1 \cdot \vec{v}_1 - 2 \hat{n} \cdot \vec{S}_2 \hat{n} \cdot \vec{a}_1 \vec{S}_1 \cdot \vec{v}_2 + \frac{3}{2} \vec{S}_2 \cdot \vec{a}_1 \vec{S}_1 \cdot \vec{v}_2 - \\ & \quad \frac{3}{2} \hat{n} \cdot \vec{a}_2 \hat{n} \cdot \vec{S}_1 \vec{S}_2 \cdot \vec{a}_1 - \frac{1}{2} \hat{n} \cdot \vec{S}_1 \hat{n} \cdot \vec{v}_2 \vec{S}_2 \cdot \vec{a}_1 + \frac{1}{4} \vec{S}_1 \cdot \vec{v}_2 \vec{S}_2 \cdot \vec{a}_1 + \frac{3}{4} \vec{S}_1 \cdot \vec{a}_2 \vec{S}_2 \cdot \vec{a}_1 - \hat{n} \cdot \vec{a}_1 \hat{n} \cdot \vec{S}_1 \vec{S}_2 \cdot \vec{a}_2 + \\ & \quad \frac{3}{2} \vec{S}_1 \cdot \vec{v}_1 \vec{S}_2 \cdot \vec{a}_2 + \frac{1}{2} \vec{S}_1 \cdot \vec{a}_1 \vec{S}_2 \cdot \vec{a}_2 - \frac{7}{2} \hat{n} \cdot \vec{S}_1 \hat{n} \cdot \vec{a}_2 \vec{S}_2 \cdot \vec{v}_1 - \frac{1}{2} \hat{n} \cdot \vec{S}_1 \hat{n} \cdot \vec{v}_2 \vec{S}_2 \cdot \vec{v}_1 + \frac{7}{4} \vec{S}_1 \cdot \vec{a}_2 \vec{S}_2 \cdot \vec{v}_1 + \\ & \quad \frac{1}{4} \vec{S}_1 \cdot \vec{v}_2 \vec{S}_2 \cdot \vec{v}_1 - \hat{n} \cdot \vec{S}_1 \hat{n} \cdot \vec{a}_1 \vec{S}_2 \cdot \vec{v}_2 + 4 \hat{n} \cdot \vec{S}_1 \hat{n} \cdot \vec{v}_2 \vec{S}_2 \cdot \vec{v}_2 + \frac{1}{2} \vec{S}_1 \cdot \vec{a}_1 \vec{S}_2 \cdot \vec{v}_2 + \frac{1}{2} \vec{S}_1 \cdot \vec{v}_1 \vec{S}_2 \cdot \vec{v}_2 - \\ & \quad 2 \vec{S}_1 \cdot \vec{v}_2 \vec{S}_2 \cdot \vec{v}_2 + \hat{n} \cdot \vec{S}_2 \hat{n} \cdot \vec{S}_1 \vec{v}_1 \cdot \vec{a}_1 + \frac{3}{2} \vec{S}_1 \cdot \vec{S}_2 \vec{v}_1 \cdot \vec{a}_1 - 3 \hat{n} \cdot \vec{S}_1 \hat{n} \cdot \vec{S}_2 \vec{v}_1 \cdot \vec{a}_2 - \frac{13}{4} \vec{S}_1 \cdot \vec{S}_2 \vec{v}_1 \cdot \vec{a}_2 + \end{aligned}$$



[illegible]

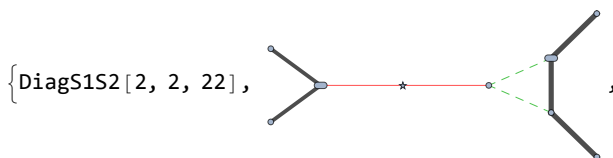

$$G^2 \left( \frac{1}{r^2} \left( -4 \hat{n} \times \vec{S_1} \cdot \vec{v_1} \hat{n} \times \vec{S_2} \cdot \vec{v_2} - 4 \hat{n} \times \vec{S_1} \cdot \vec{a_1} \hat{n} \times \vec{S_2} \cdot \vec{v_2} - 4 \hat{n} \times \vec{S_1} \cdot \vec{v_1} \hat{n} \times \vec{S_2} \cdot \vec{a_2} - \right. \right. \\ \left. \left. 4 \hat{n} \times \vec{S_1} \cdot \vec{a_1} \hat{n} \times \vec{S_2} \cdot \vec{a_2} - 2 \vec{S_1} \cdot \vec{v_2} \vec{S_2} \cdot \vec{v_1} + 2 \vec{a_1} \cdot \vec{v_2} \vec{S_1} \cdot \vec{S_2} + 2 \vec{a_1} \cdot \vec{a_2} \vec{S_1} \cdot \vec{S_2} - \right. \right. \\ \left. \left. 2 \vec{S_2} \cdot \vec{a_1} \vec{S_1} \cdot \vec{v_2} - 2 \vec{S_1} \cdot \vec{a_2} \vec{S_2} \cdot \vec{a_1} - 2 \vec{S_1} \cdot \vec{a_2} \vec{S_2} \cdot \vec{v_1} + 2 \vec{S_1} \cdot \vec{S_2} \vec{v_1} \cdot \vec{a_2} + 2 \vec{S_1} \cdot \vec{S_2} \vec{v_1} \cdot \vec{v_2} \right) + \frac{1}{r^3} \right. \\ \left. \left( 4 \hat{n} \times \vec{S_2} \cdot \vec{v_2} \vec{S_1} \times \vec{v_1} \cdot \vec{v_2} + 4 \hat{n} \times \vec{S_1} \cdot \vec{v_1} \vec{S_2} \times \vec{v_1} \cdot \vec{v_2} + 4 \hat{n} \times \vec{S_2} \cdot \vec{v_2} \vec{S_1} \times \vec{a_1} \cdot \vec{v_2} + 4 \hat{n} \times \vec{S_1} \cdot \vec{v_1} \vec{S_2} \times \vec{v_1} \cdot \vec{a_2} + \right. \right. \\ \left. \left. 16 \hat{n} \times \vec{S_2} \cdot \vec{v_2} \hat{n} \times \vec{S_1} \cdot \vec{v_1} \hat{n} \cdot \vec{v_1} + 16 \hat{n} \times \vec{S_1} \cdot \vec{v_1} \hat{n} \times \vec{S_2} \cdot \vec{a_2} \hat{n} \cdot \vec{v_1} - 16 \hat{n} \times \vec{S_1} \cdot \vec{v_1} \hat{n} \times \vec{S_2} \cdot \vec{v_2} \hat{n} \cdot \vec{v_2} - 16 \hat{n} \times \vec{S_1} \cdot \vec{a_1} \right. \right. \\ \left. \left. \hat{n} \times \vec{S_2} \cdot \vec{v_2} \hat{n} \cdot \vec{v_2} + 4 \hat{n} \cdot \vec{v_2} \vec{a_1} \cdot \vec{v_2} \vec{S_1} \cdot \vec{S_2} + 4 \hat{n} \cdot \vec{v_1} \vec{S_2} \cdot \vec{v_1} \vec{S_1} \cdot \vec{v_2} - 4 \hat{n} \cdot \vec{v_2} \vec{S_1} \cdot \vec{v_2} \vec{S_2} \cdot \vec{a_1} - 4 \hat{n} \cdot \vec{v_2} \vec{S_1} \cdot \vec{v_2} \vec{S_2} \cdot \vec{v_1} + \right. \right. \\ \left. \left. 4 \hat{n} \cdot \vec{v_1} \vec{S_1} \cdot \vec{a_2} \vec{S_2} \cdot \vec{v_1} - 4 \hat{n} \cdot \vec{v_1} \vec{S_1} \cdot \vec{S_2} \vec{v_1} \cdot \vec{a_2} + 4 \hat{n} \cdot \vec{v_2} \vec{S_1} \cdot \vec{S_2} \vec{v_1} \cdot \vec{v_2} - 4 \hat{n} \cdot \vec{v_1} \vec{S_1} \cdot \vec{S_2} \vec{v_1} \cdot \vec{v_2} \right) + \right.$$



$$\frac{1}{r^4} \left( 24 \hat{n} \times \vec{S}_1 \cdot \vec{v}_1 \hat{n} \times \vec{S}_2 \cdot \vec{v}_2 (\hat{n} \cdot \vec{v}_1)^2 + 4 \vec{S}_1 \cdot \vec{v}_2 \vec{S}_2 \cdot \vec{v}_1 (\hat{n} \cdot \vec{v}_1)^2 - 4 \vec{S}_1 \cdot \vec{S}_2 \vec{v}_1 \cdot \vec{v}_2 (\hat{n} \cdot \vec{v}_1)^2 + \right. \\ 8 \hat{n} \times \vec{S}_2 \cdot \vec{v}_2 \vec{S}_1 \times \vec{v}_1 \cdot \vec{v}_2 \hat{n} \cdot \vec{v}_1 + 8 \hat{n} \times \vec{S}_1 \cdot \vec{v}_1 \vec{S}_2 \times \vec{v}_1 \cdot \vec{v}_2 \hat{n} \cdot \vec{v}_1 - 48 \hat{n} \times \vec{S}_1 \cdot \vec{v}_1 \hat{n} \times \vec{S}_2 \cdot \vec{v}_2 \hat{n} \cdot \vec{v}_2 \hat{n} \cdot \vec{v}_1 - \\ 8 \hat{n} \cdot \vec{v}_2 \vec{S}_1 \cdot \vec{v}_2 \vec{S}_2 \cdot \vec{v}_1 \hat{n} \cdot \vec{v}_1 + 8 \hat{n} \cdot \vec{v}_2 \vec{S}_1 \cdot \vec{S}_2 \vec{v}_1 \cdot \vec{v}_2 \hat{n} \cdot \vec{v}_1 - 2 \vec{S}_1 \cdot \vec{S}_2 (\vec{v}_1 \cdot \vec{v}_2)^2 + 2 \vec{S}_1 \times \vec{v}_1 \cdot \vec{v}_2 \vec{S}_2 \times \vec{v}_1 \cdot \vec{v}_2 - \\ 8 \hat{n} \times \vec{S}_1 \cdot \vec{v}_1 \vec{S}_2 \times \vec{v}_1 \cdot \vec{v}_2 \hat{n} \cdot \vec{v}_2 - 8 \hat{n} \times \vec{S}_1 \cdot \vec{v}_1 \hat{n} \times \vec{S}_2 \cdot \vec{v}_2 \vec{v}_1 \cdot \vec{v}_1 - 2 \vec{S}_1 \cdot \vec{v}_2 \vec{S}_2 \cdot \vec{v}_1 \vec{v}_1 \cdot \vec{v}_1 + \\ \left. 8 \hat{n} \times \vec{S}_1 \cdot \vec{v}_1 \hat{n} \times \vec{S}_2 \cdot \vec{v}_2 \vec{v}_1 \cdot \vec{v}_2 + 2 \vec{S}_1 \cdot \vec{v}_2 \vec{S}_2 \cdot \vec{v}_1 \vec{v}_1 \cdot \vec{v}_2 + 2 \vec{S}_1 \cdot \vec{S}_2 \vec{v}_1 \cdot \vec{v}_1 \vec{v}_1 \cdot \vec{v}_2 \right) m_1 \}$$

$$\left\{ \text{DiagS1S2}[2, 2, 25], \right.$$

[illegible]

[illegible]



[illegible]

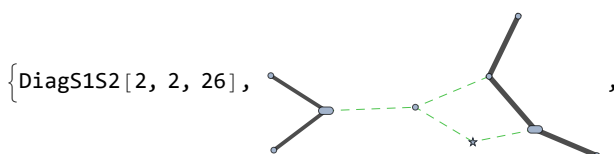

$$G^2 \left( \frac{1}{r} \left( -\frac{2}{3} \hat{n} \cdot \vec{S}_1 \hat{n} \cdot \vec{S}_2 \hat{n} \cdot \vec{a}_1 + \frac{4}{3} \hat{n} \cdot \vec{S}_1 \hat{n} \cdot \vec{S}_2 \hat{n} \cdot \vec{a}_1 - \frac{2}{3} \vec{S}_1 \cdot \vec{S}_2 \hat{n} \cdot \vec{a}_1 + \frac{1}{3} \vec{S}_1 \cdot \vec{S}_2 \hat{n} \cdot \vec{a}_1 + \frac{4}{3} \hat{n} \cdot \vec{S}_1 \hat{n} \cdot \vec{S}_2 \hat{n} \cdot \vec{v}_1 - \frac{2}{3} \hat{n} \cdot \vec{S}_1 \hat{n} \cdot \vec{S}_2 \hat{n} \cdot \vec{v}_1 - \frac{5}{3} \hat{n} \cdot \vec{v}_1 \vec{S}_1 \cdot \vec{S}_2 + \frac{1}{3} \hat{n} \cdot \vec{S}_2 \vec{S}_1 \cdot \vec{a}_1 + \hat{n} \cdot \vec{a}_1 \vec{S}_1 \cdot \vec{S}_2 + \frac{1}{3} \hat{n} \cdot \vec{S}_2 \vec{S}_1 \cdot \vec{v}_1 + \frac{1}{3} \hat{n} \cdot \vec{v}_1 \vec{S}_1 \cdot \vec{S}_2 - \frac{2}{3} \hat{n} \cdot \vec{S}_2 \vec{S}_1 \cdot \vec{a}_1 - \frac{2}{3} \hat{n} \cdot \vec{S}_2 \vec{S}_1 \cdot \vec{v}_1 + \frac{1}{3} \hat{n} \cdot \vec{S}_1 \vec{S}_2 \cdot \vec{a}_1 + \frac{1}{3} \hat{n} \cdot \vec{S}_1 \vec{S}_2 \cdot \vec{v}_1 + \frac{4}{3} \hat{n} \cdot \vec{S}_1 \vec{S}_2 \cdot \vec{v}_1 - \hat{n} \cdot \vec{S}_1 \vec{S}_2 \cdot \vec{a}_1 + \frac{1}{3} \hat{n} \cdot \vec{S}_1 \vec{S}_2 \cdot \vec{a}_1 \right) + \frac{1}{r^2} \right. \\ \left. \left( -\frac{8}{3} \hat{n} \cdot \vec{S}_1 \hat{n} \cdot \vec{S}_2 (\hat{n} \cdot \vec{a}_1)^2 - \frac{17}{6} \vec{S}_1 \cdot \vec{S}_2 (\hat{n} \cdot \vec{a}_1)^2 - \frac{2}{3} \hat{n} \cdot \vec{S}_2 \hat{n} \cdot \vec{S}_1 \hat{n} \cdot \vec{v}_1 \hat{n} \cdot \vec{a}_1 - \frac{16}{3} \hat{n} \cdot \vec{S}_1 \hat{n} \cdot \vec{S}_2 \hat{n} \cdot \vec{v}_1 \hat{n} \cdot \vec{a}_1 - \frac{8}{3} \hat{n} \cdot \vec{S}_1 \hat{n} \cdot \vec{S}_2 \hat{n} \cdot \vec{v}_2 \hat{n} \cdot \vec{a}_1 - \frac{61}{6} \hat{n} \cdot \vec{v}_1 \vec{S}_1 \cdot \vec{S}_2 \hat{n} \cdot \vec{a}_1 - \frac{4}{3} \hat{n} \cdot \vec{v}_2 \vec{S}_1 \cdot \vec{S}_2 \hat{n} \cdot \vec{a}_1 + \frac{4}{3} \hat{n} \cdot \vec{S}_2 \vec{S}_1 \cdot \vec{v}_1 \hat{n} \cdot \vec{a}_1 + \frac{2}{3} \hat{n} \cdot \vec{S}_2 \vec{S}_1 \cdot \vec{v}_2 \hat{n} \cdot \vec{a}_1 - \frac{5}{6} \hat{n} \cdot \vec{S}_1 \vec{S}_2 \cdot \vec{v}_1 \hat{n} \cdot \vec{a}_1 - \frac{4}{3} \hat{n} \cdot \vec{v}_1 \vec{S}_1 \cdot \vec{S}_2 \hat{n} \cdot \vec{a}_1 + \frac{4}{3} \hat{n} \cdot \vec{S}_2 \vec{S}_1 \cdot \vec{a}_1 \hat{n} \cdot \vec{a}_1 + \frac{1}{6} \hat{n} \cdot \vec{S}_2 \vec{S}_1 \cdot \vec{v}_1 \hat{n} \cdot \vec{a}_1 + \frac{17}{6} \hat{n} \cdot \vec{S}_1 \vec{S}_2 \cdot \vec{a}_1 \hat{n} \cdot \vec{a}_1 + \frac{41}{6} \hat{n} \cdot \vec{S}_1 \vec{S}_2 \cdot \vec{v}_1 \hat{n} \cdot \vec{a}_1 + \frac{2}{3} \hat{n} \cdot \vec{S}_1 \vec{S}_2 \cdot \vec{v}_2 \hat{n} \cdot \vec{a}_1 - \frac{14}{3} \hat{n} \cdot \vec{S}_1 \hat{n} \cdot \vec{S}_2 (\hat{n} \cdot \vec{v}_1)^2 + 2 \hat{n} \cdot \vec{S}_2 \hat{n} \cdot \vec{S}_1 (\hat{n} \cdot \vec{v}_1)^2 - \frac{8}{3} \hat{n} \cdot \vec{S}_1 \hat{n} \cdot \vec{S}_2 (\hat{n} \cdot \vec{v}_1)^2 - \frac{3}{2} \hat{n} \times \vec{S}_1 \cdot \vec{v}_1 \hat{n} \times \vec{S}_2 \cdot \vec{v}_1 + \frac{1}{2} \hat{n} \times \vec{S}_2 \cdot \vec{v}_1 \hat{n} \times \vec{S}_1 \cdot \vec{a}_1 - \frac{1}{2} \hat{n} \times \vec{S}_2 \cdot \vec{a}_1 \hat{n} \times \vec{S}_1 \cdot \vec{v}_1 - 2 \hat{n} \times \vec{S}_2 \cdot \vec{v}_1 \hat{n} \times \vec{S}_1 \cdot \vec{v}_1 + 2 \hat{n} \times \vec{S}_1 \cdot \vec{v}_1 \hat{n} \times \vec{S}_2 \cdot \vec{a}_1 - \frac{9}{2} \hat{n} \times \vec{S}_1 \cdot \vec{v}_1 \hat{n} \times \vec{S}_2 \cdot \vec{a}_1 - \frac{1}{2} \hat{n} \times \vec{S}_1 \cdot \vec{a}_1 \hat{n} \times \vec{S}_2 \cdot \vec{a}_1 - 4 \hat{n} \times \vec{S}_1 \cdot \vec{a}_1 \hat{n} \times \vec{S}_2 \cdot \vec{v}_1 + \frac{1}{2} \hat{n} \times \vec{S}_1 \cdot \vec{v}_1 \hat{n} \times \vec{S}_2 \cdot \vec{v}_1 + \frac{1}{2} \hat{n} \times \vec{S}_1 \cdot \vec{a}_1 \hat{n} \times \vec{S}_2 \cdot \vec{v}_1 - \frac{8}{3} \hat{n} \cdot \vec{S}_1 \hat{n} \cdot \vec{a}_2 \hat{n} \cdot \vec{S}_2 \hat{n} \cdot \vec{v}_1 - \frac{16}{3} \hat{n} \cdot \vec{S}_1 \hat{n} \cdot \vec{S}_2 \hat{n} \cdot \vec{v}_1 \hat{n} \cdot \vec{v}_2 + \frac{16}{3} \hat{n} \cdot \vec{S}_1 \hat{n} \cdot \vec{S}_2 \hat{n} \cdot \vec{v}_1 \hat{n} \cdot \vec{v}_2 - \frac{35}{6} (\hat{n} \cdot \vec{v}_1)^2 \vec{S}_1 \cdot \vec{S}_2 - \frac{20}{3} \hat{n} \cdot \vec{v}_1 \hat{n} \cdot \vec{v}_2 \vec{S}_1 \cdot \vec{S}_2 + \frac{4}{3} \hat{n} \cdot \vec{S}_2 \hat{n} \cdot \vec{v}_1 \vec{S}_1 \cdot \vec{a}_1 + \frac{2}{3} \hat{n} \cdot \vec{S}_2 \hat{n} \cdot \vec{v}_2 \vec{S}_1 \cdot \vec{a}_1 + \frac{2}{3} \hat{n} \cdot \vec{S}_2 \hat{n} \cdot \vec{v}_1 \vec{S}_1 \cdot \vec{a}_2 - \right. \\ \left. \right)$$

[illegible]



$$\left. \left. \left. 5 \vec{S_1} \cdot \vec{S_2} \vec{v_1} \cdot \vec{v_1} \vec{v_1} \cdot \vec{v_2} + 8 \hat{n} \times \vec{S_1} \cdot \vec{v_1} \hat{n} \times \vec{S_2} \cdot \vec{v_1} \vec{v_2} \cdot \vec{v_2} + 4 \hat{n} \cdot \vec{S_1} \hat{n} \cdot \vec{S_2} \vec{v_1} \cdot \vec{v_1} \vec{v_2} \cdot \vec{v_2} \right) \right) \right\} m_1 \Bigg\}$$

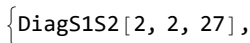

[illegible]



[illegible]

$$\begin{aligned} & 8 \hat{n} \cdot \vec{S}_1 \vec{S}_2 \cdot \vec{v}_2 \vec{v}_1 \cdot \vec{v}_2 \hat{n} \cdot \vec{v}_1 + 4 \hat{n} \cdot \vec{S}_2 \vec{S}_1 \cdot \vec{v}_1 \vec{v}_2 \cdot \vec{v}_2 \hat{n} \cdot \vec{v}_1 + 48 \hat{n} \times \vec{S}_1 \cdot \vec{v}_1 \hat{n} \times \vec{S}_2 \cdot \vec{v}_1 (\hat{n} \cdot \vec{v}_2)^2 + \\ & 4 \hat{n} \cdot \vec{S}_1 \hat{n} \cdot \vec{S}_2 (\vec{v}_1 \cdot \vec{v}_1)^2 - 2 \vec{S}_1 \cdot \vec{S}_2 (\vec{v}_1 \cdot \vec{v}_1)^2 + 4 \hat{n} \cdot \vec{S}_1 \hat{n} \cdot \vec{S}_2 (\vec{v}_1 \cdot \vec{v}_2)^2 + 4 \vec{S}_1 \times \vec{v}_1 \cdot \vec{v}_2 \vec{S}_2 \times \vec{v}_1 \cdot \vec{v}_2 - \\ & 16 \hat{n} \times \vec{S}_2 \cdot \vec{v}_1 \vec{S}_1 \times \vec{v}_1 \cdot \vec{v}_2 \hat{n} \cdot \vec{v}_2 - 16 \hat{n} \times \vec{S}_1 \cdot \vec{v}_1 \vec{S}_2 \times \vec{v}_1 \cdot \vec{v}_2 \hat{n} \cdot \vec{v}_2 + 8 (\hat{n} \cdot \vec{v}_2)^2 \vec{S}_1 \cdot \vec{v}_1 \vec{S}_2 \cdot \vec{v}_1 + \\ & 24 \hat{n} \cdot \vec{S}_1 \hat{n} \cdot \vec{S}_2 (\hat{n} \cdot \vec{v}_2)^2 \vec{v}_1 \cdot \vec{v}_1 + \frac{11}{2} \hat{n} \times \vec{S}_1 \cdot \vec{v}_1 \hat{n} \times \vec{S}_2 \cdot \vec{v}_1 \vec{v}_1 \cdot \vec{v}_1 - 8 (\hat{n} \cdot \vec{v}_2)^2 \vec{S}_1 \cdot \vec{S}_2 \vec{v}_1 \cdot \vec{v}_1 + \\ & 4 \hat{n} \cdot \vec{S}_2 \hat{n} \cdot \vec{v}_2 \vec{S}_1 \cdot \vec{v}_1 \vec{v}_1 \cdot \vec{v}_1 - 8 \hat{n} \cdot \vec{S}_2 \hat{n} \cdot \vec{v}_2 \vec{S}_1 \cdot \vec{v}_2 \vec{v}_1 \cdot \vec{v}_1 - 2 \hat{n} \cdot \vec{S}_1 \hat{n} \cdot \vec{v}_2 \vec{S}_2 \cdot \vec{v}_1 \vec{v}_1 \cdot \vec{v}_1 + \\ & \frac{1}{2} \vec{S}_1 \cdot \vec{v}_2 \vec{S}_2 \cdot \vec{v}_1 \vec{v}_1 \cdot \vec{v}_1 - 8 \hat{n} \cdot \vec{S}_1 \hat{n} \cdot \vec{v}_2 \vec{S}_2 \cdot \vec{v}_2 \vec{v}_1 \cdot \vec{v}_1 - \vec{S}_1 \cdot \vec{v}_1 \vec{S}_2 \cdot \vec{v}_2 \vec{v}_1 \cdot \vec{v}_1 + 2 \vec{S}_1 \cdot \vec{v}_2 \vec{S}_2 \cdot \vec{v}_2 \vec{v}_1 \cdot \vec{v}_1 + \\ & 2 \hat{n} \times \vec{S}_1 \cdot \vec{v}_1 \hat{n} \times \vec{S}_2 \cdot \vec{v}_1 \vec{v}_1 \cdot \vec{v}_2 + 8 \hat{n} \cdot \vec{S}_2 \hat{n} \cdot \vec{v}_2 \vec{S}_1 \cdot \vec{v}_1 \vec{v}_1 \cdot \vec{v}_2 + \frac{1}{2} \vec{S}_1 \cdot \vec{v}_1 \vec{S}_2 \cdot \vec{v}_1 \vec{v}_1 \cdot \vec{v}_2 - \\ & 2 \vec{S}_1 \cdot \vec{v}_1 \vec{S}_2 \cdot \vec{v}_2 \vec{v}_1 \cdot \vec{v}_2 + 4 \hat{n} \cdot \vec{S}_1 \hat{n} \cdot \vec{S}_2 \vec{v}_1 \cdot \vec{v}_1 \vec{v}_1 \cdot \vec{v}_2 - 2 \vec{S}_1 \cdot \vec{S}_2 \vec{v}_1 \cdot \vec{v}_1 \vec{v}_1 \cdot \vec{v}_2 - 8 \hat{n} \times \vec{S}_1 \cdot \vec{v}_1 \hat{n} \times \vec{S}_2 \cdot \vec{v}_1 \vec{v}_2 \cdot \vec{v}_2 - \\ & 2 \vec{S}_1 \cdot \vec{v}_1 \vec{S}_2 \cdot \vec{v}_1 \vec{v}_2 \cdot \vec{v}_2 - 4 \hat{n} \cdot \vec{S}_1 \hat{n} \cdot \vec{S}_2 \vec{v}_1 \cdot \vec{v}_1 \vec{v}_2 \cdot \vec{v}_2 + 2 \vec{S}_1 \cdot \vec{S}_2 \vec{v}_1 \cdot \vec{v}_1 \vec{v}_2 \cdot \vec{v}_2 \Big) \Big) m_1 \Big\} \end{aligned}$$

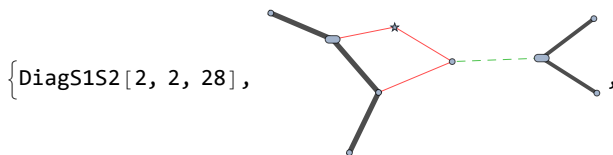

$$G^2 \left( \frac{2 \hat{n} \cdot \vec{a_1} \vec{S_1} \cdot \vec{S_2} + \hat{n} \cdot \vec{v_1} \vec{S_1} \cdot \vec{S_2} - \hat{n} \cdot \vec{S_1} \vec{S_2} \cdot \vec{a_1} - 2 \hat{n} \cdot \vec{S_1} \vec{S_2} \cdot \vec{a_1} - \hat{n} \cdot \vec{S_1} \vec{S_2} \cdot \vec{v_1} + \hat{n} \cdot \vec{a_1} \vec{S_1} \cdot \vec{S_2}}{r} + \frac{1}{r^2} \right. \\ \left( \frac{3}{2} \vec{S_1} \cdot \vec{S_2} (\hat{n} \cdot \vec{a_1})^2 - \frac{3}{2} \hat{n} \cdot \vec{v_1} \vec{S_1} \cdot \vec{S_2} \hat{n} \cdot \vec{a_1} + 4 \hat{n} \cdot \vec{v_2} \vec{S_1} \cdot \vec{S_2} \hat{n} \cdot \vec{a_1} + \frac{1}{2} \hat{n} \cdot \vec{S_1} \vec{S_2} \cdot \vec{v_1} \hat{n} \cdot \vec{a_1} - \frac{3}{2} \hat{n} \cdot \vec{S_1} \vec{S_2} \cdot \vec{a_1} \hat{n} \cdot \vec{a_1} - \right. \\ \frac{3}{2} \hat{n} \cdot \vec{S_1} \vec{S_2} \cdot \vec{v_1} \hat{n} \cdot \vec{a_1} + \frac{3}{2} \hat{n} \times \vec{S_1} \cdot \vec{v_1} \hat{n} \times \vec{S_2} \cdot \vec{v_1} + \frac{3}{2} \hat{n} \times \vec{S_2} \cdot \vec{v_1} \hat{n} \times \vec{S_1} \cdot \vec{a_1} + \frac{1}{2} \hat{n} \times \vec{S_2} \cdot \vec{a_1} \hat{n} \times \vec{S_1} \cdot \vec{v_1} + \\ \frac{1}{2} \hat{n} \times \vec{S_1} \cdot \vec{v_1} \hat{n} \times \vec{S_2} \cdot \vec{a_1} + \frac{1}{2} \hat{n} \times \vec{S_1} \cdot \vec{a_1} \hat{n} \times \vec{S_2} \cdot \vec{a_1} - \hat{n} \times \vec{S_1} \cdot \vec{a_1} \hat{n} \times \vec{S_2} \cdot \vec{v_1} - \frac{1}{2} \hat{n} \times \vec{S_1} \cdot \vec{v_1} \hat{n} \times \vec{S_2} \cdot \vec{v_1} - \\ \frac{1}{2} \hat{n} \times \vec{S_1} \cdot \vec{a_1} \hat{n} \times \vec{S_2} \cdot \vec{v_1} + \frac{1}{2} (\hat{n} \cdot \vec{v_1})^2 \vec{S_1} \cdot \vec{S_2} - \frac{3}{2} (\hat{n} \cdot \vec{v_1})^2 \vec{S_1} \cdot \vec{S_2} + 2 \hat{n} \cdot \vec{v_1} \hat{n} \cdot \vec{v_2} \vec{S_1} \cdot \vec{S_2} - \frac{1}{2} \hat{n} \cdot \vec{S_1} \hat{n} \cdot \vec{v_1} \vec{S_2} \cdot \vec{a_1} - \\ \frac{1}{2} \hat{n} \cdot \vec{S_1} \hat{n} \cdot \vec{v_1} \vec{S_2} \cdot \vec{v_1} + \vec{S_1} \cdot \vec{v_1} \vec{S_2} \cdot \vec{v_1} - 2 \vec{S_1} \cdot \vec{S_2} \vec{a_1} \cdot \vec{v_2} - \frac{3}{2} \hat{n} \cdot \vec{a_1} \hat{n} \cdot \vec{v_1} \vec{S_1} \cdot \vec{S_2} + 2 \hat{n} \cdot \vec{a_1} \hat{n} \cdot \vec{v_2} \vec{S_1} \cdot \vec{S_2} - \\ \frac{1}{2} \vec{a_1} \cdot \vec{v_2} \vec{S_1} \cdot \vec{S_2} - \vec{a_1} \cdot \vec{a_1} \vec{S_1} \cdot \vec{S_2} + \vec{S_2} \cdot \vec{a_1} \vec{S_1} \cdot \vec{v_1} + \frac{3}{2} \hat{n} \cdot \vec{S_1} \hat{n} \cdot \vec{v_1} \vec{S_2} \cdot \vec{a_1} - 2 \hat{n} \cdot \vec{S_1} \hat{n} \cdot \vec{v_2} \vec{S_2} \cdot \vec{a_1} - \vec{S_1} \cdot \vec{v_1} \vec{S_2} \cdot \vec{a_1} + \\ \vec{S_1} \cdot \vec{v_2} \vec{S_2} \cdot \vec{a_1} + 3 \hat{n} \cdot \vec{S_1} \hat{n} \cdot \vec{v_1} \vec{S_2} \cdot \vec{a_1} - 4 \hat{n} \cdot \vec{S_1} \hat{n} \cdot \vec{v_2} \vec{S_2} \cdot \vec{a_1} - 2 \vec{S_1} \cdot \vec{v_1} \vec{S_2} \cdot \vec{a_1} + 2 \vec{S_1} \cdot \vec{v_2} \vec{S_2} \cdot \vec{a_1} + \\ \vec{S_1} \cdot \vec{a_1} \vec{S_2} \cdot \vec{a_1} + \frac{3}{2} \hat{n} \cdot \vec{S_1} \hat{n} \cdot \vec{v_1} \vec{S_2} \cdot \vec{v_1} - 2 \hat{n} \cdot \vec{S_1} \hat{n} \cdot \vec{v_2} \vec{S_2} \cdot \vec{v_1} + \vec{S_1} \cdot \vec{a_1} \vec{S_2} \cdot \vec{v_1} - \vec{S_1} \cdot \vec{v_1} \vec{S_2} \cdot \vec{v_1} + \vec{S_1} \cdot \vec{v_2} \vec{S_2} \cdot \vec{v_1} + \\ \left. \vec{S_1} \cdot \vec{S_2} \vec{v_1} \cdot \vec{a_1} + \vec{S_1} \cdot \vec{S_2} \vec{v_1} \cdot \vec{a_1} - \vec{S_1} \cdot \vec{S_2} \vec{v_1} \cdot \vec{a_1} - \vec{S_1} \cdot \vec{S_2} \vec{v_1} \cdot \vec{v_1} + \vec{S_1} \cdot \vec{S_2} \vec{v_1} \cdot \vec{v_1} - \vec{S_1} \cdot \vec{S_2} \vec{v_1} \cdot \vec{v_2} \right) + \frac{1}{r^3} \\ \left( -3 \vec{S_1} \cdot \vec{S_2} (\hat{n} \cdot \vec{v_1})^3 + 2 \hat{n} \cdot \vec{v_2} \vec{S_1} \cdot \vec{S_2} (\hat{n} \cdot \vec{v_1})^2 - 3 \hat{n} \cdot \vec{a_1} \vec{S_1} \cdot \vec{S_2} (\hat{n} \cdot \vec{v_1})^2 + 3 \hat{n} \cdot \vec{S_1} \vec{S_2} \cdot \vec{a_1} (\hat{n} \cdot \vec{v_1})^2 + \right. \\ 3 \hat{n} \cdot \vec{S_1} \vec{S_2} \cdot \vec{v_1} (\hat{n} \cdot \vec{v_1})^2 - 2 \hat{n} \times \vec{S_2} \cdot \vec{v_1} \hat{n} \times \vec{S_1} \cdot \vec{v_1} \hat{n} \cdot \vec{v_1} - 2 \hat{n} \times \vec{S_1} \cdot \vec{v_1} \hat{n} \times \vec{S_2} \cdot \vec{a_1} \hat{n} \cdot \vec{v_1} - \\ 2 \hat{n} \times \vec{S_1} \cdot \vec{v_1} \hat{n} \times \vec{S_2} \cdot \vec{v_1} \hat{n} \cdot \vec{v_1} - 2 \hat{n} \times \vec{S_1} \cdot \vec{a_1} \hat{n} \times \vec{S_2} \cdot \vec{v_1} \hat{n} \cdot \vec{v_1} - \frac{1}{2} \vec{S_2} \cdot \vec{v_1} \vec{S_1} \cdot \vec{v_1} \hat{n} \cdot \vec{v_1} - \\ 2 \hat{n} \cdot \vec{S_1} \hat{n} \cdot \vec{v_2} \vec{S_2} \cdot \vec{a_1} \hat{n} \cdot \vec{v_1} - 2 \vec{S_1} \cdot \vec{v_1} \vec{S_2} \cdot \vec{a_1} \hat{n} \cdot \vec{v_1} + \frac{1}{2} \vec{S_1} \cdot \vec{v_2} \vec{S_2} \cdot \vec{a_1} \hat{n} \cdot \vec{v_1} - 2 \hat{n} \cdot \vec{S_1} \hat{n} \cdot \vec{v_2} \vec{S_2} \cdot \vec{v_1} \hat{n} \cdot \vec{v_1} - \\ 2 \vec{S_1} \cdot \vec{v_1} \vec{S_2} \cdot \vec{v_1} \hat{n} \cdot \vec{v_1} + \frac{1}{2} \vec{S_1} \cdot \vec{v_2} \vec{S_2} \cdot \vec{v_1} \hat{n} \cdot \vec{v_1} - \frac{1}{2} \vec{S_1} \cdot \vec{a_1} \vec{S_2} \cdot \vec{v_1} \hat{n} \cdot \vec{v_1} + \frac{5}{2} \vec{S_1} \cdot \vec{S_2} \vec{v_1} \cdot \vec{a_1} \hat{n} \cdot \vec{v_1} + \\ 2 \vec{S_1} \cdot \vec{S_2} \vec{v_1} \cdot \vec{v_1} \hat{n} \cdot \vec{v_1} + \vec{S_1} \cdot \vec{S_2} \vec{v_1} \cdot \vec{v_1} \hat{n} \cdot \vec{v_1} - \vec{S_1} \cdot \vec{S_2} \vec{v_1} \cdot \vec{v_2} \hat{n} \cdot \vec{v_1} - \frac{3}{2} \hat{n} \times \vec{S_2} \cdot \vec{v_1} \vec{S_1} \times \vec{v_1} \cdot \vec{v_2} -$$





[illegible]

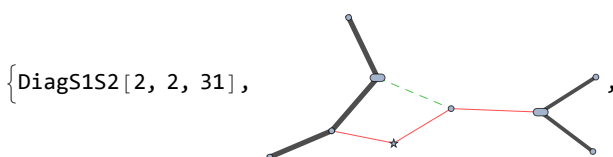

$\{\text{DiagS1S2}[2, 2, 32],$

$$G^2 \left( -\frac{(\hat{n} \cdot \vec{a}_1) \frac{1}{S_1} \cdot \frac{1}{S_2} - \frac{1}{2} \hat{n} \cdot \vec{v}_1 \frac{2}{S_1} \cdot \frac{1}{S_2} + \frac{1}{2} \hat{n} \cdot \vec{S}_1 \frac{1}{S_2} \cdot \frac{1}{\vec{a}_1} + \hat{n} \cdot \vec{S}_1 \frac{1}{S_2} \cdot \vec{a}_1 + \frac{1}{2} \hat{n} \cdot \vec{S}_1 \frac{2}{S_2} \cdot \vec{v}_1 - \frac{1}{2} \hat{n} \cdot \vec{a}_1 \frac{1}{S_1} \cdot \frac{1}{S_2}}{r} + \frac{1}{r^2} \right.$$
  

$$\left( \frac{1}{S_1} \cdot \frac{1}{S_2} (\hat{n} \cdot \vec{v}_1)^2 - \hat{n} \cdot \vec{v}_2 \frac{2}{S_1} \cdot \vec{S}_2 \hat{n} \cdot \vec{v}_1 - \hat{n} \cdot \vec{S}_1 \frac{1}{S_2} \cdot \vec{a}_1 \hat{n} \cdot \vec{v}_1 - \hat{n} \cdot \vec{S}_1 \frac{1}{S_2} \cdot \vec{v}_1 \hat{n} \cdot \vec{v}_1 + \hat{n} \cdot \vec{a}_1 \frac{1}{S_1} \cdot \frac{1}{S_2} \hat{n} \cdot \vec{v}_1 - \right.$$
  

$$\hat{n} \times \vec{S}_1 \cdot \vec{v}_1 \hat{n} \times \vec{S}_2 \cdot \vec{v}_1 - \hat{n} \times \vec{S}_2 \cdot \vec{v}_1 \hat{n} \times \vec{S}_1 \cdot \vec{a}_1 - \hat{n} \times \vec{S}_2 \cdot \vec{a}_1 \hat{n} \times \vec{S}_1 \cdot \vec{v}_1 - 2 \hat{n} \cdot \vec{a}_1 \hat{n} \cdot \vec{v}_2 \frac{1}{S_1} \cdot \vec{S}_2 + \frac{1}{S_1} \cdot \vec{S}_2 \vec{a}_1 \cdot \vec{v}_2 -$$
  

$$\frac{1}{2} \frac{1}{S_2} \cdot \vec{v}_1 \vec{S}_1 \cdot \vec{a}_1 - \hat{n} \cdot \vec{a}_1 \hat{n} \cdot \vec{v}_2 \vec{S}_1 \cdot \vec{S}_2 + \frac{1}{2} \frac{1}{\vec{a}_1} \cdot \vec{v}_2 \vec{S}_1 \cdot \vec{S}_2 + \hat{n} \cdot \vec{S}_1 \hat{n} \cdot \vec{v}_2 \vec{S}_2 \cdot \frac{1}{\vec{a}_1} - \frac{1}{2} \vec{S}_1 \cdot \vec{v}_2 \vec{S}_2 \cdot \frac{1}{\vec{a}_1} +$$
  

$$2 \hat{n} \cdot \vec{S}_1 \hat{n} \cdot \vec{v}_2 \vec{S}_2 \cdot \vec{a}_1 - \vec{S}_1 \cdot \vec{v}_2 \vec{S}_2 \cdot \vec{a}_1 + \hat{n} \cdot \vec{S}_1 \hat{n} \cdot \vec{v}_2 \vec{S}_2 \cdot \vec{v}_1 - \frac{1}{2} \frac{2}{S_1} \cdot \vec{v}_2 \vec{S}_2 \cdot \vec{v}_1 + \frac{1}{2} \vec{S}_1 \cdot \frac{1}{S_2} \vec{v}_1 \cdot \vec{a}_1 + \frac{1}{2} \frac{2}{S_1} \cdot \vec{S}_2 \vec{v}_1 \cdot \vec{v}_2 \Big) +$$
  

$$\frac{1}{r^3} \left( 4 \hat{n} \cdot \vec{v}_2 \frac{1}{S_1} \cdot \vec{S}_2 (\hat{n} \cdot \vec{v}_1)^2 + 4 \hat{n} \times \vec{S}_2 \cdot \vec{v}_1 \hat{n} \times \vec{S}_1 \cdot \vec{v}_1 \hat{n} \cdot \vec{v}_1 + 4 \hat{n} \cdot \vec{a}_1 \hat{n} \cdot \vec{v}_2 \vec{S}_1 \cdot \vec{S}_2 \hat{n} \cdot \vec{v}_1 - \vec{a}_1 \cdot \vec{v}_2 \vec{S}_1 \cdot \vec{S}_2 \hat{n} \cdot \vec{v}_1 + \right.$$
  

$$\frac{1}{S_2} \cdot \vec{v}_1 \vec{S}_1 \cdot \vec{v}_1 \hat{n} \cdot \vec{v}_1 - 4 \hat{n} \cdot \vec{S}_1 \hat{n} \cdot \vec{v}_2 \vec{S}_2 \cdot \vec{a}_1 \hat{n} \cdot \vec{v}_1 + \vec{S}_1 \cdot \vec{v}_2 \vec{S}_2 \cdot \vec{a}_1 \hat{n} \cdot \vec{v}_1 - 4 \hat{n} \cdot \vec{S}_1 \hat{n} \cdot \vec{v}_2 \vec{S}_2 \cdot \vec{v}_1 \hat{n} \cdot \vec{v}_1 +$$
  

$$\frac{1}{S_1} \cdot \vec{v}_2 \vec{S}_2 \cdot \vec{v}_1 \hat{n} \cdot \vec{v}_1 - \vec{S}_1 \cdot \frac{1}{S_2} \vec{v}_1 \cdot \vec{v}_1 \hat{n} \cdot \vec{v}_1 - 2 \vec{S}_1 \cdot \vec{S}_2 \vec{v}_1 \cdot \vec{v}_2 \hat{n} \cdot \vec{v}_1 + \hat{n} \times \vec{S}_2 \cdot \vec{v}_1 \frac{1}{S_1} \times \vec{v}_1 \cdot \vec{v}_2 + \hat{n} \times \vec{S}_2 \cdot \vec{v}_1 \vec{S}_1 \times \vec{a}_1 \cdot \vec{v}_2 +$$

$$\begin{aligned} & \hat{n} \times \vec{S}_2 \cdot \vec{a}_1 \vec{S}_1 \times \vec{v}_1 \cdot \vec{v}_2 + \hat{n} \times \vec{S}_1 \cdot \vec{v}_1 \vec{S}_2 \times \vec{a}_1 \cdot \vec{v}_2 + \hat{n} \times \vec{S}_1 \cdot \vec{v}_1 \vec{S}_2 \times \vec{v}_1 \cdot \vec{v}_2 + \hat{n} \times \vec{S}_1 \cdot \vec{a}_1 \vec{S}_2 \times \vec{v}_1 \cdot \vec{v}_2 - \\ & 4 \hat{n} \times \vec{S}_1 \cdot \vec{v}_1 \hat{n} \times \vec{S}_2 \cdot \vec{a}_1 \hat{n} \cdot \vec{v}_2 - 4 \hat{n} \times \vec{S}_1 \cdot \vec{v}_1 \hat{n} \times \vec{S}_2 \cdot \vec{v}_1 \hat{n} \cdot \vec{v}_2 - 4 \hat{n} \times \vec{S}_1 \cdot \vec{a}_1 \hat{n} \times \vec{S}_2 \cdot \vec{v}_1 \hat{n} \cdot \vec{v}_2 - \hat{n} \cdot \vec{v}_2 \vec{S}_1 \cdot \vec{a}_1 \vec{S}_2 \cdot \vec{v}_1 + \\ & \hat{n} \cdot \vec{v}_2 \vec{S}_1 \cdot \vec{S}_2 \vec{v}_1 \cdot \vec{a}_1 - \hat{n} \cdot \vec{a}_1 \vec{S}_1 \cdot \vec{S}_2 \vec{v}_1 \cdot \vec{v}_2 + \hat{n} \cdot \vec{S}_1 \vec{S}_2 \cdot \vec{a}_1 \vec{v}_1 \cdot \vec{v}_2 + \hat{n} \cdot \vec{S}_1 \vec{S}_2 \cdot \vec{v}_1 \vec{v}_1 \cdot \vec{v}_2 \Big) + \frac{1}{r^4} \\ & \left( -4 \hat{n} \times \vec{S}_2 \cdot \vec{v}_1 \vec{S}_1 \times \vec{v}_1 \cdot \vec{v}_2 \hat{n} \cdot \vec{v}_1 - 4 \hat{n} \times \vec{S}_1 \cdot \vec{v}_1 \vec{S}_2 \times \vec{v}_1 \cdot \vec{v}_2 \hat{n} \cdot \vec{v}_1 + 24 \hat{n} \times \vec{S}_1 \cdot \vec{v}_1 \hat{n} \times \vec{S}_2 \cdot \vec{v}_1 \hat{n} \cdot \vec{v}_2 \hat{n} \cdot \vec{v}_1 + \right. \\ & 4 \hat{n} \cdot \vec{v}_2 \vec{S}_1 \cdot \vec{v}_1 \vec{S}_2 \cdot \vec{v}_1 \hat{n} \cdot \vec{v}_1 - 4 \hat{n} \cdot \vec{v}_2 \vec{S}_1 \cdot \vec{S}_2 \vec{v}_1 \cdot \vec{v}_1 \hat{n} \cdot \vec{v}_1 - \\ & \left. 4 \hat{n} \times \vec{S}_1 \cdot \vec{v}_1 \hat{n} \times \vec{S}_2 \cdot \vec{v}_1 \vec{v}_1 \cdot \vec{v}_2 - \vec{S}_1 \cdot \vec{v}_1 \vec{S}_2 \cdot \vec{v}_1 \vec{v}_1 \cdot \vec{v}_2 + \vec{S}_1 \cdot \vec{S}_2 \vec{v}_1 \cdot \vec{v}_1 \vec{v}_1 \cdot \vec{v}_2 \right) \Bigg\} m_1 \Bigg\} \end{aligned}$$

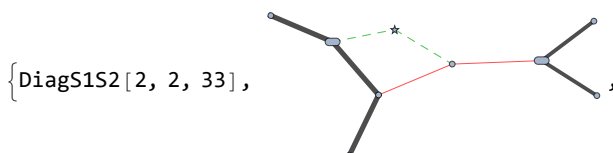

$$G^2 \left( \frac{1}{r^2} \left( 4 \hat{n} \times \vec{S}_2 \cdot \vec{a}_2 \hat{n} \times \vec{S}_1 \cdot \vec{v}_1 + 2 \hat{n} \times \vec{S}_2 \cdot \vec{v}_2 \hat{n} \times \vec{S}_1 \cdot \vec{v}_1 + 2 \hat{n} \times \vec{S}_2 \cdot \vec{a}_2 \hat{n} \times \vec{S}_1 \cdot \vec{v}_1 + 2 \hat{n} \times \vec{S}_1 \cdot \vec{a}_1 \hat{n} \times \vec{S}_2 \cdot \vec{v}_2 - \vec{S}_1 \cdot \vec{S}_2 \vec{a}_1 \cdot \vec{v}_2 + \right. \right. \\ \left. \left. 2 \vec{S}_2 \cdot \vec{v}_1 \vec{S}_1 \cdot \vec{a}_2 + \vec{S}_2 \cdot \vec{v}_1 \vec{S}_1 \cdot \vec{v}_2 + \vec{S}_1 \cdot \vec{v}_2 \vec{S}_2 \cdot \vec{a}_1 + \vec{S}_1 \cdot \vec{a}_2 \vec{S}_2 \cdot \vec{v}_1 - \vec{S}_1 \cdot \vec{S}_2 \vec{v}_1 \cdot \vec{a}_2 - 2 \vec{S}_1 \cdot \vec{S}_2 \vec{v}_1 \cdot \vec{a}_2 - \vec{S}_1 \cdot \vec{S}_2 \vec{v}_1 \cdot \vec{v}_2 \right) + \right. \\ \left. \frac{1}{r^3} \left( -2 \hat{n} \times \vec{S}_2 \cdot \vec{v}_2 \vec{S}_1 \times \vec{v}_1 \cdot \vec{a}_1 - 2 \hat{n} \times \vec{S}_2 \cdot \vec{v}_2 \vec{S}_1 \times \vec{v}_1 \cdot \vec{a}_2 - 4 \hat{n} \times \vec{S}_2 \cdot \vec{v}_2 \vec{S}_1 \times \vec{v}_1 \cdot \vec{v}_2 - 4 \hat{n} \times \vec{S}_2 \cdot \vec{a}_2 \vec{S}_1 \times \vec{v}_1 \cdot \vec{v}_2 + \right. \right. \\ \left. \left. \frac{3}{2} \hat{n} \times \vec{S}_1 \cdot \vec{v}_1 \vec{S}_2 \times \vec{a}_1 \cdot \vec{v}_2 - 3 \hat{n} \times \vec{S}_1 \cdot \vec{v}_1 \vec{S}_2 \times \vec{v}_1 \cdot \vec{v}_2 - \frac{1}{2} \hat{n} \times \vec{S}_1 \cdot \vec{a}_1 \vec{S}_2 \times \vec{v}_1 \cdot \vec{v}_2 + 2 \hat{n} \times \vec{S}_1 \cdot \vec{v}_1 \vec{S}_2 \times \vec{v}_2 \cdot \vec{a}_2 + \right. \right. \\ \left. \left. 6 \hat{n} \times \vec{S}_1 \cdot \vec{v}_1 \hat{n} \times \vec{S}_2 \cdot \vec{v}_2 \hat{n} \cdot \vec{a}_1 + 8 \hat{n} \times \vec{S}_1 \cdot \vec{v}_1 \hat{n} \times \vec{S}_2 \cdot \vec{v}_2 \hat{n} \cdot \vec{a}_2 - 12 \hat{n} \times \vec{S}_1 \cdot \vec{v}_1 \hat{n} \times \vec{S}_2 \cdot \vec{v}_2 \hat{n} \cdot \vec{v}_1 - \right. \right. \\ \left. \left. 2 \hat{n} \times \vec{S}_1 \cdot \vec{a}_1 \hat{n} \times \vec{S}_2 \cdot \vec{v}_2 \hat{n} \cdot \vec{v}_1 + 16 \hat{n} \times \vec{S}_2 \cdot \vec{v}_2 \hat{n} \times \vec{S}_1 \cdot \vec{v}_1 \hat{n} \cdot \vec{v}_2 + 16 \hat{n} \times \vec{S}_1 \cdot \vec{v}_1 \hat{n} \times \vec{S}_2 \cdot \vec{a}_2 \hat{n} \cdot \vec{v}_2 + \right. \right. \\ \left. \left. \frac{1}{2} \hat{n} \cdot \vec{v}_1 \vec{a}_1 \cdot \vec{v}_2 \vec{S}_1 \cdot \vec{S}_2 + 4 \hat{n} \cdot \vec{v}_2 \vec{S}_2 \cdot \vec{v}_1 \vec{S}_1 \cdot \vec{v}_2 - \frac{1}{2} \hat{n} \cdot \vec{v}_1 \vec{S}_1 \cdot \vec{v}_2 \vec{S}_2 \cdot \vec{a}_1 - 3 \hat{n} \cdot \vec{v}_1 \vec{S}_1 \cdot \vec{v}_2 \vec{S}_2 \cdot \vec{v}_1 + \right. \right. \\ \left. \left. 4 \hat{n} \cdot \vec{v}_2 \vec{S}_1 \cdot \vec{a}_2 \vec{S}_2 \cdot \vec{v}_1 + \frac{3}{2} \hat{n} \cdot \vec{a}_1 \vec{S}_1 \cdot \vec{v}_2 \vec{S}_2 \cdot \vec{v}_1 + 2 \hat{n} \cdot \vec{a}_2 \vec{S}_1 \cdot \vec{v}_2 \vec{S}_2 \cdot \vec{v}_1 - 4 \hat{n} \cdot \vec{v}_2 \vec{S}_1 \cdot \vec{S}_2 \vec{v}_1 \cdot \vec{a}_2 + \right. \right. \\ \left. \left. 3 \hat{n} \cdot \vec{v}_1 \vec{S}_1 \cdot \vec{S}_2 \vec{v}_1 \cdot \vec{v}_2 - 4 \hat{n} \cdot \vec{v}_2 \vec{S}_1 \cdot \vec{S}_2 \vec{v}_1 \cdot \vec{v}_2 - \frac{3}{2} \hat{n} \cdot \vec{a}_1 \vec{S}_1 \cdot \vec{S}_2 \vec{v}_1 \cdot \vec{v}_2 - 2 \hat{n} \cdot \vec{a}_2 \vec{S}_1 \cdot \vec{S}_2 \vec{v}_1 \cdot \vec{v}_2 \right) + \frac{1}{r^4} \right. \\ \left. \left( -18 \hat{n} \times \vec{S}_1 \cdot \vec{v}_1 \hat{n} \times \vec{S}_2 \cdot \vec{v}_2 (\hat{n} \cdot \vec{v}_1)^2 - 3 \vec{S}_1 \cdot \vec{v}_2 \vec{S}_2 \cdot \vec{v}_1 (\hat{n} \cdot \vec{v}_1)^2 + 3 \vec{S}_1 \cdot \vec{S}_2 \vec{v}_1 \cdot \vec{v}_2 (\hat{n} \cdot \vec{v}_1)^2 - 6 \hat{n} \times \vec{S}_1 \cdot \vec{v}_1 \right. \right. \\ \left. \left. \vec{S}_2 \times \vec{v}_1 \cdot \vec{v}_2 \hat{n} \cdot \vec{v}_1 + 48 \hat{n} \times \vec{S}_1 \cdot \vec{v}_1 \hat{n} \times \vec{S}_2 \cdot \vec{v}_2 (\hat{n} \cdot \vec{v}_2)^2 - 16 \hat{n} \times \vec{S}_2 \cdot \vec{v}_2 \vec{S}_1 \times \vec{v}_1 \cdot \vec{v}_2 \hat{n} \cdot \vec{v}_2 + 8 (\hat{n} \cdot \vec{v}_2)^2 \vec{S}_1 \cdot \vec{v}_2 \vec{S}_2 \cdot \vec{v}_1 - \right. \right. \\ \left. \left. 8 (\hat{n} \cdot \vec{v}_2)^2 \vec{S}_1 \cdot \vec{S}_2 \vec{v}_1 \cdot \vec{v}_2 - 8 \hat{n} \times \vec{S}_1 \cdot \vec{v}_1 \hat{n} \times \vec{S}_2 \cdot \vec{v}_2 \vec{v}_2 \cdot \vec{v}_2 - 2 \vec{S}_1 \cdot \vec{v}_2 \vec{S}_2 \cdot \vec{v}_1 \vec{v}_2 \cdot \vec{v}_2 + 2 \vec{S}_1 \cdot \vec{S}_2 \vec{v}_1 \cdot \vec{v}_2 \vec{v}_2 \cdot \vec{v}_2 \right) \right) m_1 \} \\$$

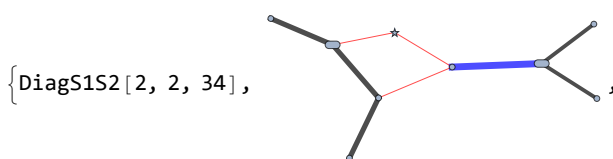

$$G^2 \left( \frac{1}{\rho^2} \left( - \left( \hat{n} \times \vec{S_1} \cdot \vec{v_1} \right) \hat{n} \times \vec{S_2} \cdot \vec{v_2} - \hat{n} \times \vec{S_1} \cdot \vec{a_1} \hat{n} \times \vec{S_2} \cdot \vec{v_2} - \hat{n} \times \vec{S_1} \cdot \vec{v_1} \hat{n} \times \vec{S_2} \cdot \vec{a_2} - \hat{n} \times \vec{S_1} \cdot \vec{a_1} \hat{n} \times \vec{S_2} \cdot \vec{a_2} - \right. \right. \\ \hat{n} \cdot \vec{v_1} \hat{n} \cdot \vec{v_2} \vec{S_1} \cdot \vec{S_2} - \hat{n} \cdot \vec{a_2} \hat{n} \cdot \vec{v_1} \vec{S_1} \cdot \vec{S_2} + \hat{n} \cdot \vec{S_1} \hat{n} \cdot \vec{v_2} \vec{S_2} \cdot \vec{a_1} + \hat{n} \cdot \vec{S_1} \hat{n} \cdot \vec{v_2} \vec{S_2} \cdot \vec{v_1} - \vec{S_1} \cdot \vec{v_2} \vec{S_2} \cdot \vec{v_1} - \\ \hat{n} \cdot \vec{a_1} \hat{n} \cdot \vec{v_2} \vec{S_1} \cdot \vec{S_2} + \vec{a_1} \cdot \vec{v_2} \vec{S_1} \cdot \vec{S_2} - \hat{n} \cdot \vec{a_1} \hat{n} \cdot \vec{a_2} \vec{S_1} \cdot \vec{S_2} + \vec{a_1} \cdot \vec{a_2} \vec{S_1} \cdot \vec{S_2} - \vec{S_2} \cdot \vec{a_1} \vec{S_1} \cdot \vec{v_2} + \\ \left. \left. \hat{n} \cdot \vec{a_2} \hat{n} \cdot \vec{S_1} \vec{S_2} \cdot \vec{a_1} - \vec{S_1} \cdot \vec{a_2} \vec{S_2} \cdot \vec{a_1} + \hat{n} \cdot \vec{S_1} \hat{n} \cdot \vec{a_2} \vec{S_2} \cdot \vec{v_1} - \vec{S_1} \cdot \vec{a_2} \vec{S_2} \cdot \vec{v_1} + \vec{S_1} \cdot \vec{S_2} \vec{v_1} \cdot \vec{a_2} + \vec{S_1} \cdot \vec{S_2} \vec{v_1} \cdot \vec{v_2} \right) \right) +$$

$$\{\text{DiagS1S2}[2, 2, 35],$$

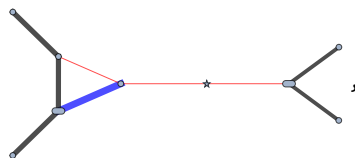

$$\begin{aligned} G^2 & \left( \frac{1}{r^2} \left( \hat{n} \times \vec{S_1} \cdot \vec{v_1} \hat{n} \times \vec{S_2} \cdot \vec{v_2} + \hat{n} \times \vec{S_1} \cdot \vec{a_1} \hat{n} \times \vec{S_2} \cdot \vec{v_2} + \hat{n} \times \vec{S_1} \cdot \vec{v_1} \hat{n} \times \vec{S_2} \cdot \vec{a_2} + \right. \right. \\ & \quad \hat{n} \times \vec{S_1} \cdot \vec{a_1} \hat{n} \times \vec{S_2} \cdot \vec{a_2} + \frac{1}{2} \vec{S_1} \cdot \vec{v_2} \vec{S_2} \cdot \vec{v_1} - \frac{1}{2} \vec{a_1} \cdot \vec{v_2} \vec{S_1} \cdot \vec{S_2} - \frac{1}{2} \vec{a_1} \cdot \vec{a_2} \vec{S_1} \cdot \vec{S_2} + \frac{1}{2} \vec{S_2} \cdot \vec{a_1} \vec{S_1} \cdot \vec{v_2} + \\ & \quad \frac{1}{2} \vec{S_1} \cdot \vec{a_2} \vec{S_2} \cdot \vec{a_1} + \frac{1}{2} \vec{S_1} \cdot \vec{a_2} \vec{S_2} \cdot \vec{v_1} - \frac{1}{2} \vec{S_1} \cdot \vec{S_2} \vec{v_1} \cdot \vec{a_2} - \frac{1}{2} \vec{S_1} \cdot \vec{S_2} \vec{v_1} \cdot \vec{v_2} \Big) + \frac{1}{r^3} \\ & \quad \left( - \left( \hat{n} \times \vec{S_2} \cdot \vec{v_2} \right) \vec{S_1} \times \vec{v_1} \cdot \vec{v_2} - \hat{n} \times \vec{S_1} \cdot \vec{v_1} \vec{S_2} \times \vec{v_1} \cdot \vec{v_2} - \hat{n} \times \vec{S_2} \cdot \vec{v_2} \vec{S_1} \times \vec{a_1} \cdot \vec{v_2} - \hat{n} \times \vec{S_1} \cdot \vec{v_1} \vec{S_2} \times \vec{v_1} \cdot \vec{a_2} - \right. \\ & \quad \left. 4 \hat{n} \times \vec{S_2} \cdot \vec{v_2} \hat{n} \times \vec{S_1} \cdot \vec{v_1} \hat{n} \cdot \vec{v_1} - 4 \hat{n} \times \vec{S_1} \cdot \vec{v_1} \hat{n} \times \vec{S_2} \cdot \vec{a_2} \hat{n} \cdot \vec{v_1} + 4 \hat{n} \times \vec{S_1} \cdot \vec{v_1} \hat{n} \times \vec{S_2} \cdot \vec{v_2} \hat{n} \cdot \vec{v_2} + \right. \end{aligned}$$

$$\begin{aligned} & 4 \hat{n} \cdot \vec{S}_1 \cdot \vec{a}_1 \hat{n} \cdot \vec{S}_2 \cdot \vec{v}_2 \hat{n} \cdot \vec{v}_2 - \hat{n} \cdot \vec{v}_2 \vec{a}_1 \cdot \vec{v}_2 \vec{S}_1 \cdot \vec{S}_2 - \hat{n} \cdot \vec{v}_1 \vec{S}_2 \cdot \vec{v}_1 \vec{S}_1 \cdot \vec{v}_2 + \hat{n} \cdot \vec{v}_2 \vec{S}_1 \cdot \vec{v}_2 \vec{S}_2 \cdot \vec{a}_1 + \\ & \hat{n} \cdot \vec{v}_2 \vec{S}_1 \cdot \vec{v}_2 \vec{S}_2 \cdot \vec{v}_1 - \hat{n} \cdot \vec{v}_1 \vec{S}_1 \cdot \vec{a}_2 \vec{S}_2 \cdot \vec{v}_1 + \hat{n} \cdot \vec{v}_1 \vec{S}_1 \cdot \vec{S}_2 \vec{v}_1 \cdot \vec{a}_2 - \hat{n} \cdot \vec{v}_2 \vec{S}_1 \cdot \vec{S}_2 \vec{v}_1 \cdot \vec{v}_2 + \hat{n} \cdot \vec{v}_1 \vec{S}_1 \cdot \vec{S}_2 \vec{v}_1 \cdot \vec{v}_2 \Big) + \\ & \frac{1}{\rho^4} \Big( - \left( \vec{S}_1 \cdot \vec{S}_2 \right) \left( \vec{v}_1 \cdot \vec{v}_2 \right)^2 + 4 \hat{n} \cdot \vec{S}_1 \cdot \vec{v}_1 \hat{n} \cdot \vec{S}_2 \cdot \vec{v}_2 \vec{v}_1 \cdot \vec{v}_2 + 4 \hat{n} \cdot \vec{v}_1 \hat{n} \cdot \vec{v}_2 \vec{S}_1 \cdot \vec{S}_2 \vec{v}_1 \cdot \vec{v}_2 + \\ & \vec{S}_1 \cdot \vec{v}_2 \vec{S}_2 \cdot \vec{v}_1 \vec{v}_1 \cdot \vec{v}_2 + \vec{S}_1 \times \vec{v}_1 \cdot \vec{v}_2 \vec{S}_2 \times \vec{v}_1 \cdot \vec{v}_2 + 4 \hat{n} \times \vec{S}_2 \cdot \vec{v}_2 \vec{S}_1 \times \vec{v}_1 \cdot \vec{v}_2 \hat{n} \cdot \vec{v}_1 - \\ & 4 \hat{n} \times \vec{S}_1 \cdot \vec{v}_1 \vec{S}_2 \times \vec{v}_1 \cdot \vec{v}_2 \hat{n} \cdot \vec{v}_2 - 24 \hat{n} \times \vec{S}_1 \cdot \vec{v}_1 \hat{n} \times \vec{S}_2 \cdot \vec{v}_2 \hat{n} \cdot \vec{v}_1 \hat{n} \cdot \vec{v}_2 - 4 \hat{n} \cdot \vec{v}_1 \hat{n} \cdot \vec{v}_2 \vec{S}_1 \cdot \vec{v}_2 \vec{S}_2 \cdot \vec{v}_1 \Big) \Big) m_1 \Big\} \end{aligned}$$

$$\{\text{DiagS1S2}[2, 2, 36],$$

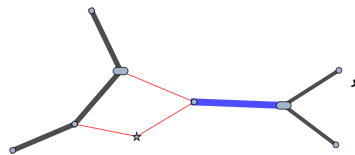

[illegible]

$$\{\text{DiagS1S2}[2, 2, 37],$$

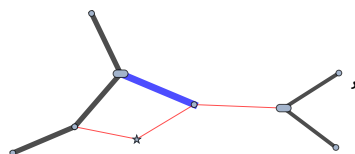

$$G^2 \left( \frac{1}{r^3} \left( 3 \hat{n} \times \vec{S}_1 \cdot \vec{v}_1 \vec{S}_2 \times \vec{v}_1 \cdot \vec{v}_2 - 2 \hat{n} \times \vec{S}_2 \cdot \vec{v}_2 \vec{S}_1 \times \vec{v}_1 \cdot \vec{a}_1 + \frac{5}{2} \hat{n} \times \vec{S}_1 \cdot \vec{v}_1 \vec{S}_2 \times \vec{a}_1 \cdot \vec{v}_2 + 3 \hat{n} \times \vec{S}_1 \cdot \vec{v}_1 \vec{S}_2 \times \vec{v}_1 \cdot \vec{a}_2 + \right. \right.$$

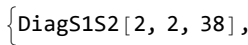

[illegible]

[illegible]

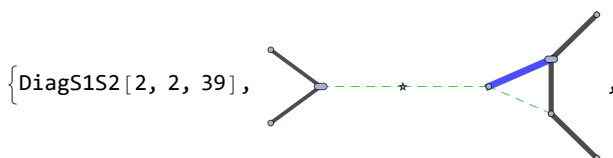

$$G^2 \left( \frac{1}{r^2} \left( - \left( \frac{1}{\vec{S}_1} \cdot \frac{1}{\vec{S}_2} \right) (\hat{n} \cdot \vec{v}_1)^2 + \hat{n} \cdot \vec{S}_1 \vec{S}_2 \cdot \vec{a}_1 \hat{n} \cdot \vec{v}_1 + \hat{n} \cdot \vec{S}_1 \vec{S}_2 \cdot \vec{v}_1 \hat{n} \cdot \vec{v}_1 - 2 \hat{n} \cdot \vec{a}_1 \vec{S}_1 \cdot \vec{S}_2 \hat{n} \cdot \vec{v}_1 - 4 \hat{n} \times \vec{S}_1 \cdot \vec{v}_1 \hat{n} \times \vec{S}_2 \cdot \vec{v}_1 - \right. \right. \\ \left. \left. 4 \hat{n} \times \vec{S}_2 \cdot \vec{v}_1 \hat{n} \times \vec{S}_1 \cdot \vec{a}_1 - 4 \hat{n} \times \vec{S}_2 \cdot \vec{a}_1 \hat{n} \times \vec{S}_1 \cdot \vec{v}_1 + \hat{n} \cdot \vec{a}_1 \hat{n} \cdot \vec{S}_1 \vec{S}_2 \cdot \vec{v}_1 - \frac{5}{2} \vec{S}_1 \cdot \vec{v}_1 \vec{S}_2 \cdot \vec{v}_1 - \frac{5}{2} \vec{S}_2 \cdot \vec{v}_1 \vec{S}_1 \cdot \vec{a}_1 - \right. \right.$$

$$\{\text{DiagS1S2}[2, 2, 40],$$

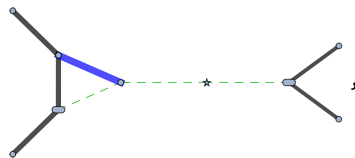

$$\begin{aligned} G^2 \left( \frac{1}{r^2} \right. & \left( 4 \hat{n} \cdot \vec{S}_1 \hat{n} \cdot \vec{S}_2 \left( \hat{n} \cdot \vec{v}_1 \right)^2 + 8 \hat{n} \cdot \vec{S}_2 \hat{n} \cdot \vec{a}_1 \hat{n} \cdot \vec{S}_1 \hat{n} \cdot \vec{v}_1 - 2 \hat{n} \cdot \vec{S}_2 \vec{S}_1 \cdot \vec{v}_1 \hat{n} \cdot \vec{v}_1 - 2 \hat{n} \cdot \vec{S}_2 \vec{S}_1 \cdot \vec{a}_1 \hat{n} \cdot \vec{v}_1 + \right. \\ & \hat{n} \times \vec{S}_1 \cdot \vec{v}_1 \hat{n} \times \vec{S}_2 \cdot \vec{v}_1 + \hat{n} \times \vec{S}_2 \cdot \vec{v}_1 \hat{n} \times \vec{S}_1 \cdot \vec{a}_1 + \hat{n} \times \vec{S}_2 \cdot \vec{a}_1 \hat{n} \times \vec{S}_1 \cdot \vec{v}_1 + \frac{1}{2} \vec{S}_1 \cdot \vec{v}_1 \vec{S}_2 \cdot \vec{v}_1 + \\ & \left. \frac{1}{2} \vec{S}_2 \cdot \vec{v}_1 \vec{S}_1 \cdot \vec{a}_1 - 2 \hat{n} \cdot \vec{S}_2 \hat{n} \cdot \vec{a}_1 \vec{S}_1 \cdot \vec{v}_1 + \frac{1}{2} \vec{S}_2 \cdot \vec{a}_1 \vec{S}_1 \cdot \vec{v}_1 - \vec{S}_1 \cdot \vec{S}_2 \vec{v}_1 \cdot \vec{a}_1 - \frac{1}{2} \vec{S}_1 \cdot \vec{S}_2 \vec{v}_1 \cdot \vec{v}_1 \right) + \\ & \left. \frac{1}{r^3} \left( -24 \hat{n} \cdot \vec{S}_2 \hat{n} \cdot \vec{S}_1 \left( \hat{n} \cdot \vec{v}_1 \right)^3 + 24 \hat{n} \cdot \vec{S}_1 \hat{n} \cdot \vec{S}_2 \hat{n} \cdot \vec{v}_2 \left( \hat{n} \cdot \vec{v}_1 \right)^2 - 4 \hat{n} \cdot \vec{S}_2 \vec{S}_1 \cdot \vec{v}_2 \left( \hat{n} \cdot \vec{v}_1 \right)^2 + \right. \right. \\ & 4 \hat{n} \cdot \vec{S}_1 \vec{S}_2 \cdot \vec{v}_1 \left( \hat{n} \cdot \vec{v}_1 \right)^2 + 12 \hat{n} \cdot \vec{S}_2 \vec{S}_1 \cdot \vec{v}_1 \left( \hat{n} \cdot \vec{v}_1 \right)^2 - 4 \hat{n} \cdot \vec{S}_1 \vec{S}_2 \cdot \vec{v}_2 \left( \hat{n} \cdot \vec{v}_1 \right)^2 - \\ & 4 \hat{n} \times \vec{S}_2 \cdot \vec{v}_1 \hat{n} \times \vec{S}_1 \cdot \vec{v}_1 \hat{n} \cdot \vec{v}_1 + 48 \hat{n} \cdot \vec{a}_1 \hat{n} \cdot \vec{S}_1 \hat{n} \cdot \vec{S}_2 \hat{n} \cdot \vec{v}_2 \hat{n} \cdot \vec{v}_1 - 8 \hat{n} \cdot \vec{S}_2 \hat{n} \cdot \vec{v}_2 \vec{S}_1 \cdot \vec{v}_1 \hat{n} \cdot \vec{v}_1 - \\ & 8 \hat{n} \cdot \vec{S}_1 \hat{n} \cdot \vec{S}_2 \vec{a}_1 \cdot \vec{v}_2 \hat{n} \cdot \vec{v}_1 - 8 \hat{n} \cdot \vec{S}_2 \hat{n} \cdot \vec{v}_2 \vec{S}_1 \cdot \vec{a}_1 \hat{n} \cdot \vec{v}_1 - 3 \vec{S}_2 \cdot \vec{v}_1 \vec{S}_1 \cdot \vec{v}_1 \hat{n} \cdot \vec{v}_1 - 8 \hat{n} \cdot \vec{a}_1 \hat{n} \cdot \vec{S}_2 \vec{S}_1 \cdot \vec{v}_2 \hat{n} \cdot \vec{v}_1 - \\ & 8 \hat{n} \cdot \vec{a}_1 \hat{n} \cdot \vec{S}_1 \vec{S}_2 \cdot \vec{v}_2 \hat{n} \cdot \vec{v}_1 + 2 \vec{S}_1 \cdot \vec{v}_1 \vec{S}_2 \cdot \vec{v}_2 \hat{n} \cdot \vec{v}_1 + 2 \vec{S}_1 \cdot \vec{a}_1 \vec{S}_2 \cdot \vec{v}_2 \hat{n} \cdot \vec{v}_1 + 8 \hat{n} \cdot \vec{S}_2 \hat{n} \cdot \vec{S}_1 \vec{v}_1 \cdot \vec{v}_1 \hat{n} \cdot \vec{v}_1 + \\ & \vec{S}_1 \cdot \vec{S}_2 \vec{v}_1 \cdot \vec{v}_1 \hat{n} \cdot \vec{v}_1 - 8 \hat{n} \cdot \vec{S}_1 \hat{n} \cdot \vec{S}_2 \vec{v}_1 \cdot \vec{v}_2 \hat{n} \cdot \vec{v}_1 - \hat{n} \times \vec{S}_2 \cdot \vec{v}_1 \vec{S}_1 \times \vec{v}_1 \cdot \vec{v}_2 - \hat{n} \times \vec{S}_2 \cdot \vec{v}_1 \vec{S}_1 \times \vec{a}_1 \cdot \vec{v}_2 - \\ & \hat{n} \times \vec{S}_2 \cdot \vec{a}_1 \vec{S}_1 \times \vec{v}_1 \cdot \vec{v}_2 - \hat{n} \times \vec{S}_1 \cdot \vec{v}_1 \vec{S}_2 \times \vec{a}_1 \cdot \vec{v}_2 - \hat{n} \times \vec{S}_1 \cdot \vec{v}_1 \vec{S}_2 \times \vec{v}_1 \cdot \vec{v}_2 - \hat{n} \times \vec{S}_1 \cdot \vec{a}_1 \vec{S}_2 \times \vec{v}_1 \cdot \vec{v}_2 + \\ & 4 \hat{n} \times \vec{S}_1 \cdot \vec{v}_1 \hat{n} \times \vec{S}_2 \cdot \vec{a}_1 \hat{n} \cdot \vec{v}_2 + 4 \hat{n} \times \vec{S}_1 \cdot \vec{v}_1 \hat{n} \times \vec{S}_2 \cdot \vec{v}_1 \hat{n} \cdot \vec{v}_2 + 4 \hat{n} \times \vec{S}_1 \cdot \vec{a}_1 \hat{n} \times \vec{S}_2 \cdot \vec{v}_1 \hat{n} \cdot \vec{v}_2 - \\ & \left. 8 \hat{n} \cdot \vec{a}_1 \hat{n} \cdot \vec{S}_2 \hat{n} \cdot \vec{v}_2 \vec{S}_1 \cdot \vec{v}_1 + 2 \hat{n} \cdot \vec{S}_2 \vec{a}_1 \cdot \vec{v}_2 \vec{S}_1 \cdot \vec{v}_1 + \hat{n} \cdot \vec{v}_2 \vec{S}_1 \cdot \vec{v}_1 \vec{S}_2 \cdot \vec{a}_1 + \hat{n} \cdot \vec{v}_2 \vec{S}_1 \cdot \vec{v}_1 \vec{S}_2 \cdot \vec{v}_1 + \right. \end{aligned}$$



$$\begin{aligned} & \hat{n} \cdot \vec{v}_2 \vec{S}_1 \cdot \vec{a}_1 \vec{S}_2 \cdot \vec{v}_1 + 2 \hat{n} \cdot \vec{a}_1 \vec{S}_1 \cdot \vec{v}_1 \vec{S}_2 \cdot \vec{v}_2 - 2 \hat{n} \cdot \vec{v}_2 \vec{S}_1 \cdot \vec{S}_2 \vec{v}_1 \cdot \vec{a}_1 - \hat{n} \cdot \vec{v}_2 \vec{S}_1 \cdot \vec{S}_2 \vec{v}_1 \cdot \vec{v}_1 - \\ & 2 \hat{n} \cdot \vec{S}_2 \vec{S}_1 \cdot \vec{v}_1 \vec{v}_1 \cdot \vec{v}_1 - 8 \hat{n} \cdot \vec{a}_1 \hat{n} \cdot \vec{S}_1 \hat{n} \cdot \vec{S}_2 \vec{v}_1 \cdot \vec{v}_2 + 2 \hat{n} \cdot \vec{S}_2 \vec{S}_1 \cdot \vec{v}_1 \vec{v}_1 \cdot \vec{v}_2 + 2 \hat{n} \cdot \vec{S}_2 \vec{S}_1 \cdot \vec{a}_1 \vec{v}_1 \cdot \vec{v}_2 \Big) + \\ & \frac{1}{\kappa^4} \Big( -192 \hat{n} \cdot \vec{S}_1 \hat{n} \cdot \vec{S}_2 \hat{n} \cdot \vec{v}_2 \left( \hat{n} \cdot \vec{v}_1 \right)^3 + 24 \hat{n} \cdot \vec{S}_2 \vec{S}_1 \cdot \vec{v}_2 \left( \hat{n} \cdot \vec{v}_1 \right)^3 + 24 \hat{n} \cdot \vec{S}_1 \vec{S}_2 \cdot \vec{v}_2 \left( \hat{n} \cdot \vec{v}_1 \right)^3 + \\ & 72 \hat{n} \cdot \vec{S}_2 \hat{n} \cdot \vec{v}_2 \vec{S}_1 \cdot \vec{v}_1 \left( \hat{n} \cdot \vec{v}_1 \right)^2 + 24 \hat{n} \cdot \vec{S}_1 \hat{n} \cdot \vec{v}_2 \vec{S}_2 \cdot \vec{v}_1 \left( \hat{n} \cdot \vec{v}_1 \right)^2 - 4 \vec{S}_1 \cdot \vec{v}_2 \vec{S}_2 \cdot \vec{v}_1 \left( \hat{n} \cdot \vec{v}_1 \right)^2 - \\ & 12 \vec{S}_1 \cdot \vec{v}_1 \vec{S}_2 \cdot \vec{v}_2 \left( \hat{n} \cdot \vec{v}_1 \right)^2 + 72 \hat{n} \cdot \vec{S}_1 \hat{n} \cdot \vec{S}_2 \vec{v}_1 \cdot \vec{v}_2 \left( \hat{n} \cdot \vec{v}_1 \right)^2 + 4 \hat{n} \times \vec{S}_2 \cdot \vec{v}_1 \vec{S}_1 \times \vec{v}_1 \cdot \vec{v}_2 \hat{n} \cdot \vec{v}_1 + \\ & 4 \hat{n} \times \vec{S}_1 \cdot \vec{v}_1 \vec{S}_2 \times \vec{v}_1 \cdot \vec{v}_2 \hat{n} \cdot \vec{v}_1 - 24 \hat{n} \times \vec{S}_1 \cdot \vec{v}_1 \hat{n} \times \vec{S}_2 \cdot \vec{v}_1 \hat{n} \cdot \vec{v}_2 \hat{n} \cdot \vec{v}_1 - 12 \hat{n} \cdot \vec{v}_2 \vec{S}_1 \cdot \vec{v}_1 \vec{S}_2 \cdot \vec{v}_1 \hat{n} \cdot \vec{v}_1 + \\ & 48 \hat{n} \cdot \vec{S}_1 \hat{n} \cdot \vec{S}_2 \hat{n} \cdot \vec{v}_2 \vec{v}_1 \cdot \vec{v}_1 \hat{n} \cdot \vec{v}_1 + 4 \hat{n} \cdot \vec{v}_2 \vec{S}_1 \cdot \vec{S}_2 \vec{v}_1 \cdot \vec{v}_1 \hat{n} \cdot \vec{v}_1 - 8 \hat{n} \cdot \vec{S}_2 \vec{S}_1 \cdot \vec{v}_2 \vec{v}_1 \cdot \vec{v}_1 \hat{n} \cdot \vec{v}_1 - \\ & 8 \hat{n} \cdot \vec{S}_1 \vec{S}_2 \cdot \vec{v}_2 \vec{v}_1 \cdot \vec{v}_1 \hat{n} \cdot \vec{v}_1 - 24 \hat{n} \cdot \vec{S}_2 \vec{S}_1 \cdot \vec{v}_1 \vec{v}_1 \cdot \vec{v}_2 \hat{n} \cdot \vec{v}_1 - 8 \hat{n} \cdot \vec{S}_1 \vec{S}_2 \cdot \vec{v}_1 \vec{v}_1 \cdot \vec{v}_2 \hat{n} \cdot \vec{v}_1 - \\ & 8 \hat{n} \cdot \vec{S}_2 \hat{n} \cdot \vec{v}_2 \vec{S}_1 \cdot \vec{v}_1 \vec{v}_1 \cdot \vec{v}_1 + 2 \vec{S}_1 \cdot \vec{v}_1 \vec{S}_2 \cdot \vec{v}_2 \vec{v}_1 \cdot \vec{v}_1 + 4 \hat{n} \times \vec{S}_1 \cdot \vec{v}_1 \hat{n} \times \vec{S}_2 \cdot \vec{v}_1 \vec{v}_1 \cdot \vec{v}_2 + \\ & 3 \vec{S}_1 \cdot \vec{v}_1 \vec{S}_2 \cdot \vec{v}_1 \vec{v}_1 \cdot \vec{v}_2 - 8 \hat{n} \cdot \vec{S}_1 \hat{n} \cdot \vec{S}_2 \vec{v}_1 \cdot \vec{v}_1 \vec{v}_1 \cdot \vec{v}_2 - \vec{S}_1 \cdot \vec{S}_2 \vec{v}_1 \cdot \vec{v}_1 \vec{v}_1 \cdot \vec{v}_2 \Big) \Big) m_1 \} \end{aligned}$$

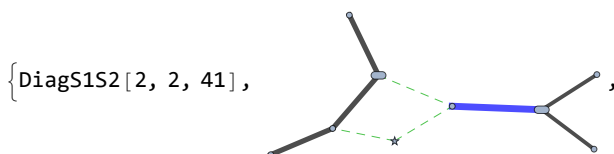

[illegible]

$$\{\text{DiagS1S2}[2, 2, 42],$$

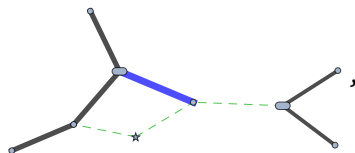

$$G^2 \left( \frac{1}{r^2} \left( 2 \vec{S_1} \cdot \vec{S_2} (\hat{n} \cdot \vec{a_1})^2 + 2 \hat{n} \cdot \vec{v_1} \vec{S_1} \cdot \vec{S_2} \hat{n} \cdot \vec{a_1} - 6 \hat{n} \cdot \vec{S_1} \vec{S_2} \cdot \vec{v_1} \hat{n} \cdot \vec{a_1} + 2 \hat{n} \cdot \vec{v_1} \vec{S_1} \cdot \vec{S_2} \hat{n} \cdot \vec{a_1} - 2 \hat{n} \cdot \vec{S_1} \vec{S_2} \cdot \vec{a_1} \hat{n} \cdot \vec{a_1} - \right. \right.$$

[illegible]

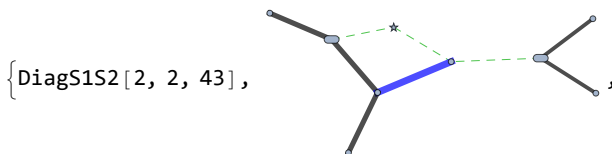

$$G^2 \left( \frac{1}{r^2} \left( \frac{8}{3} \hat{n} \cdot \vec{S}_1 \hat{n} \cdot \vec{S}_2 (\hat{n} \cdot \vec{v}_1)^2 + \frac{16}{3} \vec{S}_1 \cdot \vec{S}_2 (\hat{n} \cdot \vec{v}_1)^2 + \frac{16}{3} \hat{n} \cdot \vec{S}_1 \hat{n} \cdot \vec{a}_1 \hat{n} \cdot \vec{S}_2 \hat{n} \cdot \vec{v}_1 - \right. \right. \\ \left. \frac{4}{3} \hat{n} \cdot \vec{S}_2 \vec{S}_1 \cdot \vec{a}_1 \hat{n} \cdot \vec{v}_1 + \frac{32}{3} \hat{n} \cdot \vec{a}_1 \vec{S}_1 \cdot \vec{S}_2 \hat{n} \cdot \vec{v}_1 - \frac{4}{3} \hat{n} \cdot \vec{S}_2 \vec{S}_1 \cdot \vec{v}_1 \hat{n} \cdot \vec{v}_1 - \frac{16}{3} \hat{n} \cdot \vec{S}_1 \vec{S}_2 \cdot \vec{v}_1 \hat{n} \cdot \vec{v}_1 - \right. \\ \left. \frac{16}{3} \hat{n} \cdot \vec{S}_1 \vec{S}_2 \cdot \vec{a}_1 \hat{n} \cdot \vec{v}_1 + 6 \hat{n} \times \vec{S}_1 \cdot \vec{v}_1 \hat{n} \times \vec{S}_2 \cdot \vec{v}_1 + 6 \hat{n} \times \vec{S}_1 \cdot \vec{v}_1 \hat{n} \times \vec{S}_2 \cdot \vec{a}_1 + 6 \hat{n} \times \vec{S}_1 \cdot \vec{a}_1 \hat{n} \times \vec{S}_2 \cdot \vec{v}_1 - \right.$$

$$\begin{aligned} & \frac{4}{3} \hat{n} \cdot \vec{a}_1 \hat{n} \cdot \vec{S}_2 \vec{S}_1 \cdot \vec{v}_1 + \frac{17}{3} \vec{S}_1 \cdot \vec{v}_1 \vec{S}_2 \cdot \vec{v}_1 + \frac{17}{3} \vec{S}_1 \cdot \vec{v}_1 \vec{S}_2 \cdot \vec{a}_1 - \frac{16}{3} \hat{n} \cdot \vec{S}_1 \hat{n} \cdot \vec{a}_1 \vec{S}_2 \cdot \vec{v}_1 + \frac{17}{3} \vec{S}_1 \cdot \vec{a}_1 \vec{S}_2 \cdot \vec{v}_1 + \\ & \left( \frac{32}{3} \hat{n} \cdot \vec{S}_1 \hat{n} \cdot \vec{S}_2 \vec{v}_1 \cdot \vec{a}_1 - \frac{34}{3} \vec{S}_1 \cdot \vec{S}_2 \vec{v}_1 \cdot \vec{a}_1 + \frac{16}{3} \hat{n} \cdot \vec{S}_1 \hat{n} \cdot \vec{S}_2 \vec{v}_1 \cdot \vec{v}_1 - \frac{17}{3} \vec{S}_1 \cdot \vec{S}_2 \vec{v}_1 \cdot \vec{v}_1 \right) + \frac{1}{r^3} \\ & \left( -12 \hat{n} \cdot \vec{S}_2 \hat{n} \cdot \vec{S}_1 (\hat{n} \cdot \vec{v}_1)^3 - 4 \hat{n} \cdot \vec{S}_1 \hat{n} \cdot \vec{S}_2 (\hat{n} \cdot \vec{v}_1)^3 - \frac{34}{3} \vec{S}_1 \cdot \vec{S}_2 (\hat{n} \cdot \vec{v}_1)^3 - 10 \vec{S}_1 \cdot \vec{S}_2 (\hat{n} \cdot \vec{v}_1)^3 - \right. \\ & 24 \hat{n} \cdot \vec{a}_1 \hat{n} \cdot \vec{S}_1 \hat{n} \cdot \vec{S}_2 (\hat{n} \cdot \vec{v}_1)^2 + 16 \hat{n} \cdot \vec{S}_1 \hat{n} \cdot \vec{S}_2 \hat{n} \cdot \vec{v}_2 (\hat{n} \cdot \vec{v}_1)^2 + \frac{64}{3} \hat{n} \cdot \vec{v}_2 \vec{S}_1 \cdot \vec{S}_2 (\hat{n} \cdot \vec{v}_1)^2 + \\ & 2 \hat{n} \cdot \vec{S}_2 \vec{S}_1 \cdot \vec{v}_1 (\hat{n} \cdot \vec{v}_1)^2 - \frac{8}{3} \hat{n} \cdot \vec{S}_2 \vec{S}_1 \cdot \vec{v}_2 (\hat{n} \cdot \vec{v}_1)^2 + 12 \hat{n} \cdot \vec{S}_1 \vec{S}_2 \cdot \vec{v}_1 (\hat{n} \cdot \vec{v}_1)^2 + 4 \hat{n} \cdot \vec{S}_2 \vec{S}_1 \cdot \vec{a}_1 (\hat{n} \cdot \vec{v}_1)^2 - \\ & 20 \hat{n} \cdot \vec{a}_1 \vec{S}_1 \cdot \vec{S}_2 (\hat{n} \cdot \vec{v}_1)^2 + 6 \hat{n} \cdot \vec{S}_2 \vec{S}_1 \cdot \vec{v}_1 (\hat{n} \cdot \vec{v}_1)^2 + 8 \hat{n} \cdot \vec{S}_1 \vec{S}_2 \cdot \vec{a}_1 (\hat{n} \cdot \vec{v}_1)^2 + 12 \hat{n} \cdot \vec{S}_1 \vec{S}_2 \cdot \vec{v}_1 (\hat{n} \cdot \vec{v}_1)^2 - \\ & \frac{8}{3} \hat{n} \cdot \vec{S}_1 \vec{S}_2 \cdot \vec{v}_2 (\hat{n} \cdot \vec{v}_1)^2 - 12 \hat{n} \times \vec{S}_2 \cdot \vec{v}_1 \hat{n} \times \vec{S}_1 \cdot \vec{v}_1 \hat{n} \cdot \vec{v}_1 - 14 \hat{n} \times \vec{S}_1 \cdot \vec{v}_1 \hat{n} \times \vec{S}_2 \cdot \vec{a}_1 \hat{n} \cdot \vec{v}_1 - \\ & 12 \hat{n} \times \vec{S}_1 \cdot \vec{v}_1 \hat{n} \times \vec{S}_2 \cdot \vec{v}_1 \hat{n} \cdot \vec{v}_1 - 10 \hat{n} \times \vec{S}_1 \cdot \vec{a}_1 \hat{n} \times \vec{S}_2 \cdot \vec{v}_1 \hat{n} \cdot \vec{v}_1 - \frac{16}{3} \hat{n} \cdot \vec{S}_2 \hat{n} \cdot \vec{v}_2 \vec{S}_1 \cdot \vec{v}_1 \hat{n} \cdot \vec{v}_1 + \\ & 8 \hat{n} \cdot \vec{a}_1 \hat{n} \cdot \vec{S}_2 \vec{S}_1 \cdot \vec{v}_1 \hat{n} \cdot \vec{v}_1 - 9 \vec{S}_2 \cdot \vec{v}_1 \vec{S}_1 \cdot \vec{v}_1 \hat{n} \cdot \vec{v}_1 - \frac{13}{2} \vec{S}_1 \cdot \vec{v}_1 \vec{S}_2 \cdot \vec{a}_1 \hat{n} \cdot \vec{v}_1 + 16 \hat{n} \cdot \vec{a}_1 \hat{n} \cdot \vec{S}_1 \vec{S}_2 \cdot \vec{v}_1 \hat{n} \cdot \vec{v}_1 - \\ & \frac{64}{3} \hat{n} \cdot \vec{S}_1 \hat{n} \cdot \vec{v}_2 \vec{S}_2 \cdot \vec{v}_1 \hat{n} \cdot \vec{v}_1 - 9 \vec{S}_1 \cdot \vec{v}_1 \vec{S}_2 \cdot \vec{v}_1 \hat{n} \cdot \vec{v}_1 + \frac{16}{3} \vec{S}_1 \cdot \vec{v}_2 \vec{S}_2 \cdot \vec{v}_1 \hat{n} \cdot \vec{v}_1 - \\ & \frac{15}{2} \vec{S}_1 \cdot \vec{a}_1 \vec{S}_2 \cdot \vec{v}_1 \hat{n} \cdot \vec{v}_1 + \frac{4}{3} \vec{S}_1 \cdot \vec{v}_1 \vec{S}_2 \cdot \vec{v}_2 \hat{n} \cdot \vec{v}_1 - 14 \hat{n} \cdot \vec{S}_1 \hat{n} \cdot \vec{S}_2 \vec{v}_1 \cdot \vec{a}_1 \hat{n} \cdot \vec{v}_1 + 15 \vec{S}_1 \cdot \vec{S}_2 \vec{v}_1 \cdot \vec{a}_1 \hat{n} \cdot \vec{v}_1 - \\ & 4 \hat{n} \cdot \vec{S}_2 \hat{n} \cdot \vec{S}_1 \vec{v}_1 \cdot \vec{v}_1 \hat{n} \cdot \vec{v}_1 - 12 \hat{n} \cdot \vec{S}_1 \hat{n} \cdot \vec{S}_2 \vec{v}_1 \cdot \vec{v}_1 \hat{n} \cdot \vec{v}_1 + 12 \vec{S}_1 \cdot \vec{S}_2 \vec{v}_1 \cdot \vec{v}_1 \hat{n} \cdot \vec{v}_1 + \\ & 10 \vec{S}_1 \cdot \vec{S}_2 \vec{v}_1 \cdot \vec{v}_1 \hat{n} \cdot \vec{v}_1 - \frac{16}{3} \hat{n} \cdot \vec{S}_1 \hat{n} \cdot \vec{S}_2 \vec{v}_1 \cdot \vec{v}_2 \hat{n} \cdot \vec{v}_1 - \frac{32}{3} \vec{S}_1 \cdot \vec{S}_2 \vec{v}_1 \cdot \vec{v}_2 \hat{n} \cdot \vec{v}_1 - 6 \hat{n} \times \vec{S}_2 \cdot \vec{v}_1 \vec{S}_1 \times \vec{v}_1 \cdot \vec{v}_2 - \\ & 3 \hat{n} \times \vec{S}_2 \cdot \vec{v}_1 \vec{S}_1 \times \vec{v}_1 \cdot \vec{a}_1 - \frac{7}{2} \hat{n} \times \vec{S}_1 \cdot \vec{v}_1 \vec{S}_2 \times \vec{v}_1 \cdot \vec{a}_1 - 6 \hat{n} \times \vec{S}_1 \cdot \vec{v}_1 \vec{S}_2 \times \vec{v}_1 \cdot \vec{v}_2 + 24 \hat{n} \times \vec{S}_1 \cdot \vec{v}_1 \hat{n} \times \vec{S}_2 \cdot \vec{v}_1 \hat{n} \cdot \vec{v}_2 + \\ & \frac{34}{3} \hat{n} \cdot \vec{v}_2 \vec{S}_1 \cdot \vec{v}_1 \vec{S}_2 \cdot \vec{v}_1 - 4 \hat{n} \cdot \vec{a}_1 \vec{S}_1 \cdot \vec{v}_1 \vec{S}_2 \cdot \vec{v}_1 + \frac{7}{2} \hat{n} \cdot \vec{S}_2 \vec{S}_1 \cdot \vec{v}_1 \vec{v}_1 \cdot \vec{a}_1 + \frac{5}{2} \hat{n} \cdot \vec{S}_1 \vec{S}_2 \cdot \vec{v}_1 \vec{v}_1 \cdot \vec{a}_1 + \\ & 6 \hat{n} \cdot \vec{a}_1 \hat{n} \cdot \vec{S}_1 \hat{n} \cdot \vec{S}_2 \vec{v}_1 \cdot \vec{v}_1 + \frac{64}{3} \hat{n} \cdot \vec{S}_1 \hat{n} \cdot \vec{S}_2 \hat{n} \cdot \vec{v}_2 \vec{v}_1 \cdot \vec{v}_1 - \frac{34}{3} \hat{n} \cdot \vec{v}_2 \vec{S}_1 \cdot \vec{S}_2 \vec{v}_1 \cdot \vec{v}_1 + 3 \hat{n} \cdot \vec{S}_2 \vec{S}_1 \cdot \vec{v}_1 \vec{v}_1 \cdot \vec{v}_1 - \\ & \frac{16}{3} \hat{n} \cdot \vec{S}_2 \vec{S}_1 \cdot \vec{v}_2 \vec{v}_1 \cdot \vec{v}_1 - \frac{3}{2} \hat{n} \cdot \vec{S}_2 \vec{S}_1 \cdot \vec{a}_1 \vec{v}_1 \cdot \vec{v}_1 + 5 \hat{n} \cdot \vec{a}_1 \vec{S}_1 \cdot \vec{S}_2 \vec{v}_1 \cdot \vec{v}_1 + \hat{n} \cdot \vec{S}_2 \vec{S}_1 \cdot \vec{v}_1 \vec{v}_1 \cdot \vec{v}_1 - \\ & \frac{5}{2} \hat{n} \cdot \vec{S}_1 \vec{S}_2 \cdot \vec{a}_1 \vec{v}_1 \cdot \vec{v}_1 - \frac{16}{3} \hat{n} \cdot \vec{S}_1 \vec{S}_2 \cdot \vec{v}_2 \vec{v}_1 \cdot \vec{v}_1 + \frac{4}{3} \hat{n} \cdot \vec{S}_2 \vec{S}_1 \cdot \vec{v}_1 \vec{v}_1 \cdot \vec{v}_2 + \frac{16}{3} \hat{n} \cdot \vec{S}_1 \vec{S}_2 \cdot \vec{v}_1 \vec{v}_1 \cdot \vec{v}_2 \Big) + \frac{1}{r^4} \\ & \left( 16 \hat{n} \cdot \vec{S}_1 \hat{n} \cdot \vec{S}_2 (\hat{n} \cdot \vec{v}_1)^4 + 16 \vec{S}_1 \cdot \vec{S}_2 (\hat{n} \cdot \vec{v}_1)^4 - 96 \hat{n} \cdot \vec{S}_1 \hat{n} \cdot \vec{S}_2 \hat{n} \cdot \vec{v}_2 (\hat{n} \cdot \vec{v}_1)^3 - 60 \hat{n} \cdot \vec{v}_2 \vec{S}_1 \cdot \vec{S}_2 (\hat{n} \cdot \vec{v}_1)^3 - \right. \\ & 8 \hat{n} \cdot \vec{S}_2 \vec{S}_1 \cdot \vec{v}_1 (\hat{n} \cdot \vec{v}_1)^3 + 12 \hat{n} \cdot \vec{S}_2 \vec{S}_1 \cdot \vec{v}_2 (\hat{n} \cdot \vec{v}_1)^3 - 20 \hat{n} \cdot \vec{S}_1 \vec{S}_2 \cdot \vec{v}_1 (\hat{n} \cdot \vec{v}_1)^3 + 12 \hat{n} \cdot \vec{S}_1 \vec{S}_2 \cdot \vec{v}_2 (\hat{n} \cdot \vec{v}_1)^3 + \\ & 18 \hat{n} \times \vec{S}_1 \cdot \vec{v}_1 \hat{n} \times \vec{S}_2 \cdot \vec{v}_1 (\hat{n} \cdot \vec{v}_1)^2 + 36 \hat{n} \cdot \vec{S}_2 \hat{n} \cdot \vec{v}_2 \vec{S}_1 \cdot \vec{v}_1 (\hat{n} \cdot \vec{v}_1)^2 + 72 \hat{n} \cdot \vec{S}_1 \hat{n} \cdot \vec{v}_2 \vec{S}_2 \cdot \vec{v}_1 (\hat{n} \cdot \vec{v}_1)^2 + \\ & 13 \vec{S}_1 \cdot \vec{v}_1 \vec{S}_2 \cdot \vec{v}_1 (\hat{n} \cdot \vec{v}_1)^2 - 12 \vec{S}_1 \cdot \vec{v}_2 \vec{S}_2 \cdot \vec{v}_1 (\hat{n} \cdot \vec{v}_1)^2 - 6 \vec{S}_1 \cdot \vec{v}_1 \vec{S}_2 \cdot \vec{v}_2 (\hat{n} \cdot \vec{v}_1)^2 + \\ & 12 \hat{n} \cdot \vec{S}_1 \hat{n} \cdot \vec{S}_2 \vec{v}_1 \cdot \vec{v}_1 (\hat{n} \cdot \vec{v}_1)^2 - 21 \vec{S}_1 \cdot \vec{S}_2 \vec{v}_1 \cdot \$$

$$\{\text{DiagS1S2}[2, 2, 44],$$

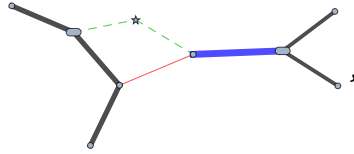

[illegible]

[illegible]

$$\left. \begin{aligned} & 2 \hat{n} \cdot \vec{S}_2 \hat{n} \cdot \vec{v}_2 \vec{S}_1 \cdot \vec{v}_1 \vec{v}_1 \cdot \vec{v}_2 + 2 \hat{n} \cdot \vec{S}_1 \hat{n} \cdot \vec{v}_2 \vec{S}_2 \cdot \vec{v}_1 \vec{v}_1 \cdot \vec{v}_2 - \frac{1}{2} \vec{S}_1 \cdot \vec{v}_2 \vec{S}_2 \cdot \vec{v}_1 \vec{v}_1 \cdot \vec{v}_2 + \vec{S}_1 \cdot \vec{v}_1 \vec{S}_2 \cdot \vec{v}_2 \vec{v}_1 \cdot \vec{v}_2 - \\ & \vec{S}_1 \cdot \vec{S}_2 \vec{v}_1 \cdot \vec{v}_1 \vec{v}_1 \cdot \vec{v}_2 - \frac{1}{2} \vec{S}_1 \cdot \vec{v}_1 \vec{S}_2 \cdot \vec{v}_1 \vec{v}_2 \cdot \vec{v}_2 + 2 \hat{n} \cdot \vec{S}_1 \hat{n} \cdot \vec{S}_2 \vec{v}_1 \cdot \vec{v}_1 \vec{v}_2 \cdot \vec{v}_2 + \frac{1}{2} \vec{S}_1 \cdot \vec{S}_2 \vec{v}_1 \cdot \vec{v}_1 \vec{v}_2 \cdot \vec{v}_2 \end{aligned} \right) \Bigg) m_1 \Bigg\}$$

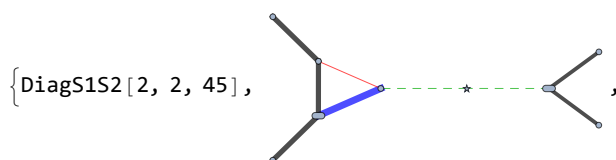

[illegible]







[illegible]

[illegible]

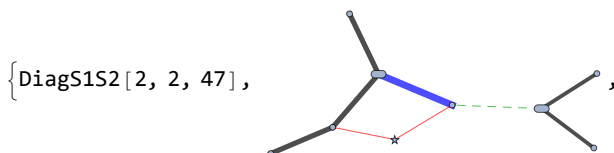

[illegible]



$$\begin{aligned}
& 16 \hat{n} \cdot \vec{S}_1 \hat{n} \cdot \vec{S}_2 \hat{n} \cdot \vec{v}_2 \vec{v}_1 \cdot \vec{v}_2 \hat{n} \cdot \vec{v}_1 - \frac{32}{3} \hat{n} \cdot \vec{v}_2 \vec{S}_1 \cdot \vec{S}_2 \vec{v}_1 \cdot \vec{v}_2 \hat{n} \cdot \vec{v}_1 + 6 \hat{n} \cdot \vec{S}_2 \vec{S}_1 \cdot \vec{v}_1 \vec{v}_1 \cdot \vec{v}_2 \hat{n} \cdot \vec{v}_1 - \\
& \frac{8}{3} \hat{n} \cdot \vec{S}_2 \vec{S}_1 \cdot \vec{v}_2 \vec{v}_1 \cdot \vec{v}_2 \hat{n} \cdot \vec{v}_1 - 4 \hat{n} \cdot \vec{S}_1 \vec{S}_2 \cdot \vec{v}_1 \vec{v}_1 \cdot \vec{v}_2 \hat{n} \cdot \vec{v}_1 - \frac{8}{3} \hat{n} \cdot \vec{S}_1 \vec{S}_2 \cdot \vec{v}_2 \vec{v}_1 \cdot \vec{v}_2 \hat{n} \cdot \vec{v}_1 - \\
& \frac{4}{3} \hat{n} \cdot \vec{S}_2 \vec{S}_1 \cdot \vec{v}_1 \vec{v}_2 \cdot \vec{v}_2 \hat{n} \cdot \vec{v}_1 + \frac{8}{3} \hat{n} \cdot \vec{S}_1 \vec{S}_2 \cdot \vec{v}_1 \vec{v}_2 \cdot \vec{v}_2 \hat{n} \cdot \vec{v}_1 - 48 \hat{n} \times \vec{S}_1 \cdot \vec{v}_1 \hat{n} \times \vec{S}_2 \cdot \vec{v}_1 (\hat{n} \cdot \vec{v}_2)^2 - \\
& 4 \hat{n} \cdot \vec{S}_1 \hat{n} \cdot \vec{S}_2 (\vec{v}_1 \cdot \vec{v}_1)^2 - \frac{4}{3} \hat{n} \cdot \vec{S}_1 \hat{n} \cdot \vec{S}_2 (\vec{v}_1 \cdot \vec{v}_2)^2 + \frac{4}{3} \vec{S}_1 \cdot \vec{S}_2 (\vec{v}_1 \cdot \vec{v}_2)^2 - 4 \vec{S}_1 \times \vec{v}_1 \cdot \vec{v}_2 \vec{S}_2 \times \vec{v}_1 \cdot \vec{v}_2 + \\
& 16 \hat{n} \times \vec{S}_2 \cdot \vec{v}_1 \vec{S}_1 \times \vec{v}_1 \cdot \vec{v}_2 \hat{n} \cdot \vec{v}_2 + 16 \hat{n} \times \vec{S}_1 \cdot \vec{v}_1 \vec{S}_2 \times \vec{v}_1 \cdot \vec{v}_2 \hat{n} \cdot \vec{v}_2 - \frac{16}{3} (\hat{n} \cdot \vec{v}_2)^2 \vec{S}_1 \cdot \vec{v}_1 \vec{S}_2 \cdot \vec{v}_1 + \\
& 40 \hat{n} \cdot \vec{S}_1 \hat{n} \cdot \vec{S}_2 (\hat{n} \cdot \vec{v}_2)^2 \vec{v}_1 \cdot \vec{v}_1 + 4 \hat{n} \times \vec{S}_1 \cdot \vec{v}_1 \hat{n} \times \vec{S}_2 \cdot \vec{v}_1 \vec{v}_1 \cdot \vec{v}_1 + \frac{16}{3} (\hat{n} \cdot \vec{v}_2)^2 \vec{S}_1 \cdot \vec{S}_2 \vec{v}_1 \cdot \vec{v}_1 + \\
& 12 \hat{n} \cdot \vec{S}_2 \hat{n} \cdot \vec{v}_2 \vec{S}_1 \cdot \vec{v}_1 \vec{v}_1 \cdot \vec{v}_1 - \frac{40}{3} \hat{n} \cdot \vec{S}_2 \hat{n} \cdot \vec{v}_2 \vec{S}_1 \cdot \vec{v}_2 \vec{v}_1 \cdot \vec{v}_1 + 4 \hat{n} \cdot \vec{S}_1 \hat{n} \cdot \vec{v}_2 \vec{S}_2 \cdot \vec{v}_1 \vec{v}_1 \cdot \vec{v}_1 + \\
& 2 \vec{S}_1 \cdot \vec{v}_1 \vec{S}_2 \cdot \vec{v}_1 \vec{v}_1 \cdot \vec{v}_1 - \vec{S}_1 \cdot \vec{v}_2 \vec{S}_2 \cdot \vec{v}_1 \vec{v}_1 \cdot \vec{v}_1 - \frac{40}{3} \hat{n} \cdot \vec{S}_1 \hat{n} \cdot \vec{v}_2 \vec{S}_2 \cdot \vec{v}_2 \vec{v}_1 \cdot \vec{v}_1 - 3 \vec{S}_1 \cdot \vec{v}_1 \vec{S}_2 \cdot \vec{v}_2 \vec{v}_1 \cdot \vec{v}_1 + \\
& \frac{10}{3} \vec{S}_1 \cdot \vec{v}_2 \vec{S}_2 \cdot \vec{v}_2 \vec{v}_1 \cdot \vec{v}_1 - 8 \hat{n} \times \vec{S}_1 \cdot \vec{v}_1 \hat{n} \times \vec{S}_2 \cdot \vec{v}_1 \vec{v}_1 \cdot \vec{v}_2 - \frac{8}{3} \hat{n} \cdot \vec{S}_2 \hat{n} \cdot \vec{v}_2 \vec{S}_1 \cdot \vec{v}_1 \vec{v}_1 \cdot \vec{v}_2 + \\
& \frac{16}{3} \hat{n} \cdot \vec{S}_1 \hat{n} \cdot \vec{v}_2 \vec{S}_2 \cdot \vec{v}_1 \vec{v}_1 \cdot \vec{v}_2 - \vec{S}_1 \cdot \vec{v}_1 \vec{S}_2 \cdot \vec{v}_1 \vec{v}_1 \cdot \vec{v}_2 - \frac{4}{3} \vec{S}_1 \cdot \vec{v}_2 \vec{S}_2 \cdot \vec{v}_1 \vec{v}_1 \cdot \vec{v}_2 + \frac{2}{3} \vec{S}_1 \cdot \vec{v}_1 \vec{S}_2 \cdot \vec{v}_2 \vec{v}_1 \cdot \vec{v}_2 + \\
& 12 \hat{n} \cdot \vec{S}_1 \hat{n} \cdot \vec{S}_2 \vec{v}_1 \cdot \vec{v}_1 \vec{v}_1 \cdot \vec{v}_2 - \vec{S}_1 \cdot \vec{S}_2 \vec{v}_1 \cdot \vec{v}_1 \vec{v}_1 \cdot \vec{v}_2 + 8 \hat{n} \times \vec{S}_1 \cdot \vec{v}_1 \hat{n} \times \vec{S}_2 \cdot \vec{v}_1 \vec{v}_2 \cdot \vec{v}_2 + \\
& \frac{4}{3} \vec{S}_1 \cdot \vec{v}_1 \vec{S}_2 \cdot \vec{v}_1 \vec{v}_2 \cdot \vec{v}_2 - \frac{20}{3} \hat{n} \cdot \vec{S}_1 \hat{n} \cdot \vec{S}_2 \vec{v}_1 \cdot \vec{v}_1 \vec{v}_2 \cdot \vec{v}_2 - \frac{4}{3} \vec{S}_1 \cdot \vec{S}_2 \vec{v}_1 \cdot \vec{v}_1 \vec{v}_2 \cdot \vec{v}_2 \Big) \Big) m_1 \Big\}
\end{aligned}$$

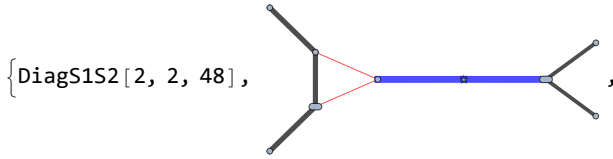

$$\begin{aligned}
& G^2 \left( \frac{1}{r^2} \left( \hat{n} \times \vec{S}_1 \cdot \vec{v}_1 \hat{n} \times \vec{S}_2 \cdot \vec{v}_2 + \hat{n} \times \vec{S}_1 \cdot \vec{a}_1 \hat{n} \times \vec{S}_2 \cdot \vec{v}_2 + \hat{n} \times \vec{S}_1 \cdot \vec{v}_1 \hat{n} \times \vec{S}_2 \cdot \vec{a}_2 + \right. \right. \\
& \hat{n} \times \vec{S}_1 \cdot \vec{a}_1 \hat{n} \times \vec{S}_2 \cdot \vec{a}_2 + \frac{1}{2} \vec{S}_1 \cdot \vec{v}_2 \vec{S}_2 \cdot \vec{v}_1 - \frac{1}{2} \vec{a}_1 \cdot \vec{v}_2 \vec{S}_1 \cdot \vec{S}_2 - \frac{1}{2} \vec{a}_1 \cdot \vec{a}_2 \vec{S}_1 \cdot \vec{S}_2 + \frac{1}{2} \vec{S}_2 \cdot \vec{a}_1 \vec{S}_1 \cdot \vec{v}_2 + \\
& \frac{1}{2} \vec{S}_1 \cdot \vec{a}_2 \vec{S}_2 \cdot \vec{a}_1 + \frac{1}{2} \vec{S}_1 \cdot \vec{a}_2 \vec{S}_2 \cdot \vec{v}_1 - \frac{1}{2} \vec{S}_1 \cdot \vec{S}_2 \vec{v}_1 \cdot \vec{a}_2 - \frac{1}{2} \vec{S}_1 \cdot \vec{S}_2 \vec{v}_1 \cdot \vec{v}_2 \Big) + \frac{1}{r^3} \\
& \left( - (\hat{n} \times \vec{S}_2 \cdot \vec{v}_2) \vec{S}_1 \times \vec{v}_1 \cdot \vec{v}_2 - \hat{n} \times \vec{S}_1 \cdot \vec{v}_1 \vec{S}_2 \times \vec{v}_1 \cdot \vec{v}_2 - \hat{n} \times \vec{S}_2 \cdot \vec{v}_2 \vec{S}_1 \times \vec{a}_1 \cdot \vec{v}_2 - \hat{n} \times \vec{S}_1 \cdot \vec{v}_1 \vec{S}_2 \times \vec{v}_1 \cdot \vec{a}_2 - \right. \\
& 4 \hat{n} \times \vec{S}_2 \cdot \vec{v}_2 \hat{n} \times \vec{S}_1 \cdot \vec{v}_1 \hat{n} \cdot \vec{v}_1 - 4 \hat{n} \times \vec{S}_1 \cdot \vec{v}_1 \hat{n} \times \vec{S}_2 \cdot \vec{a}_2 \hat{n} \cdot \vec{v}_1 + 4 \hat{n} \times \vec{S}_1 \cdot \vec{v}_1 \hat{n} \times \vec{S}_2 \cdot \vec{v}_2 \hat{n} \cdot \vec{v}_2 + \\
& 4 \hat{n} \times \vec{S}_1 \cdot \vec{a}_1 \hat{n} \times \vec{S}_2 \cdot \vec{v}_2 \hat{n} \cdot \vec{v}_2 - \hat{n} \cdot \vec{v}_2 \vec{a}_1 \cdot \vec{v}_2 \vec{S}_1 \cdot \vec{S}_2 - \hat{n} \cdot \vec{v}_1 \vec{S}_2 \cdot \vec{v}_1 \vec{S}_1 \cdot \vec{v}_2 + \hat{n} \cdot \vec{v}_2 \vec{S}_1 \cdot \vec{v}_2 \vec{S}_2 \cdot \vec{a}_1 + \\
& \hat{n} \cdot \vec{v}_2 \vec{S}_1 \cdot \vec{v}_2 \vec{S}_2 \cdot \vec{v}_1 - \hat{n} \cdot \vec{v}_1 \vec{S}_1 \cdot \vec{a}_2 \vec{S}_2 \cdot \vec{v}_1 + \hat{n} \cdot \vec{v}_1 \vec{S}_1 \cdot \vec{S}_2 \vec{v}_1 \cdot \vec{a}_2 - \hat{n} \cdot \vec{v}_2 \vec{S}_1 \cdot \vec{S}_2 \vec{v}_1 \cdot \vec{v}_2 + \hat{n} \cdot \vec{v}_1 \vec{S}_1 \cdot \vec{S}_2 \vec{v}_1 \cdot \vec{v}_2 \Big) + \\
& \frac{1}{r^4} \left( - (\vec{S}_1 \cdot \vec{S}_2) (\vec{v}_1 \cdot \vec{v}_2)^2 + 4 \hat{n} \times \vec{S}_1 \cdot \vec{v}_1 \hat{n} \times \vec{S}_2 \cdot \vec{v}_2 \vec{v}_1 \cdot \vec{v}_2 + 4 \hat{n} \cdot \vec{v}_1 \hat{n} \cdot \vec{v}_2 \vec{S}_1 \cdot \vec{S}_2 \vec{v}_1 \cdot \vec{v}_2 + \right. \\
& \vec{S}_1 \cdot \vec{v}_2 \vec{S}_2 \cdot \vec{v}_1 \vec{v}_1 \cdot \vec{v}_2 + \vec{S}_1 \times \vec{v}_1 \cdot \vec{v}_2 \vec{S}_2 \times \vec{v}_1 \cdot \vec{v}_2 + 4 \hat{n} \times \vec{S}_2 \cdot \vec{v}_2 \vec{S}_1 \times \vec{v}_1 \cdot \vec{v}_2 \hat{n} \cdot \vec{v}_1 - \\
& 4 \hat{n} \times \vec{S}_1 \cdot \vec{v}_1 \vec{S}_2 \times \vec{v}_1 \cdot \vec{v}_2 \hat{n} \cdot \vec{v}_2 - 24 \hat{n} \times \vec{S}_1 \cdot \vec{v}_1 \hat{n} \times \vec{S}_2 \cdot \vec{v}_2 \hat{n} \cdot \vec{v}_1 \hat{n} \cdot \vec{v}_2 - 4 \hat{n} \cdot \vec{v}_1 \hat{n} \cdot \vec{v}_2 \vec{S}_1 \cdot \vec{v}_2 \vec{S}_2 \cdot \vec{v}_1 \Big) \Big) m_1 \Big\}
\end{aligned}$$

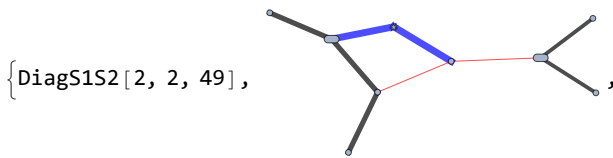

$$G^2 \left( \frac{1}{r^2} \left( -2 \hat{n} \times \vec{S}_1 \cdot \vec{v}_1 \hat{n} \times \vec{S}_2 \cdot \vec{v}_2 - 2 \hat{n} \times \vec{S}_1 \cdot \vec{a}_1 \hat{n} \times \vec{S}_2 \cdot \vec{v}_2 - 2 \hat{n} \times \vec{S}_1 \cdot \vec{v}_1 \hat{n} \times \vec{S}_2 \cdot \vec{a}_2 - 2 \hat{n} \times \vec{S}_1 \cdot \vec{a}_1 \hat{n} \times \vec{S}_2 \cdot \vec{a}_2 - \frac{1}{\vec{S}_1} \cdot \vec{v}_2 \frac{1}{\vec{S}_2} \cdot \vec{v}_1 + \right. \right. \\ \left. \vec{a}_1 \cdot \vec{v}_2 \vec{S}_1 \cdot \vec{S}_2 + \vec{a}_1 \cdot \vec{a}_2 \vec{S}_1 \cdot \vec{S}_2 - \frac{1}{\vec{S}_2} \cdot \vec{a}_1 \vec{S}_1 \cdot \vec{v}_2 - \vec{S}_1 \cdot \vec{a}_2 \vec{S}_2 \cdot \vec{a}_1 - \frac{1}{\vec{S}_1} \cdot \vec{a}_2 \vec{S}_2 \cdot \vec{v}_1 + \frac{1}{\vec{S}_1} \cdot \vec{S}_2 \vec{v}_1 \cdot \vec{a}_2 + \frac{1}{\vec{S}_1} \cdot \frac{1}{\vec{S}_2} \vec{v}_1 \cdot \vec{v}_2 \right) + \\ \frac{1}{r^3} \left( 2 \hat{n} \times \vec{S}_2 \cdot \vec{v}_2 \frac{1}{\vec{S}_1} \times \vec{v}_1 \cdot \vec{v}_2 - 3 \hat{n} \times \vec{S}_1 \cdot \vec{v}_1 \frac{1}{\vec{S}_2} \times \vec{v}_1 \cdot \vec{v}_2 + 2 \hat{n} \times \vec{S}_2 \cdot \vec{v}_2 \vec{S}_1 \times \vec{a}_1 \cdot \vec{v}_2 - 2 \hat{n} \times \vec{S}_2 \cdot \vec{v}_2 \vec{S}_1 \times \vec{v}_1 \cdot \vec{a}_1 + \right. \\ \frac{7}{2} \hat{n} \times \vec{S}_1 \cdot \vec{v}_1 \vec{S}_2 \times \vec{a}_1 \cdot \vec{v}_2 - 3 \hat{n} \times \vec{S}_1 \cdot \vec{v}_1 \vec{S}_2 \times \vec{v}_1 \cdot \vec{a}_2 + 5 \hat{n} \times \vec{S}_1 \cdot \vec{v}_1 \vec{S}_2 \times \vec{v}_1 \cdot \vec{v}_2 + \frac{3}{2} \hat{n} \times \vec{S}_1 \cdot \vec{a}_1 \vec{S}_2 \times \vec{v}_1 \cdot \vec{v}_2 + \\ 14 \hat{n} \times \vec{S}_1 \cdot \vec{v}_1 \hat{n} \times \vec{S}_2 \cdot \vec{v}_2 \hat{n} \cdot \vec{a}_1 - 12 \hat{n} \times \vec{S}_2 \cdot \vec{v}_2 \hat{n} \times \vec{S}_1 \cdot \vec{v}_1 \hat{n} \cdot \vec{v}_1 - 12 \hat{n} \times \vec{S}_1 \cdot \vec{v}_1 \hat{n} \times \vec{S}_2 \cdot \vec{a}_2 \hat{n} \cdot \vec{v}_1 + \\ 20 \hat{n} \times \vec{S}_1 \cdot \vec{v}_1 \hat{n} \times \vec{S}_2 \cdot \vec{v}_2 \hat{n} \cdot \vec{v}_1 + 6 \hat{n} \times \vec{S}_1 \cdot \vec{a}_1 \hat{n} \times \vec{S}_2 \cdot \vec{v}_2 \hat{n} \cdot \vec{v}_1 - 8 \hat{n} \times \vec{S}_1 \cdot \vec{v}_1 \hat{n} \times \vec{S}_2 \cdot \vec{v}_2 \hat{n} \cdot \vec{v}_2 - \\ 8 \hat{n} \times \vec{S}_1 \cdot \vec{a}_1 \hat{n} \times \vec{S}_2 \cdot \vec{v}_2 \hat{n} \cdot \vec{v}_2 - \frac{3}{2} \hat{n} \cdot \vec{v}_1 \vec{a}_1 \cdot \vec{v}_2 \vec{S}_1 \cdot \vec{S}_2 + 2 \hat{n} \cdot \vec{v}_2 \vec{a}_1 \cdot \vec{v}_2 \vec{S}_1 \cdot \vec{S}_2 - \\ 3 \hat{n} \cdot \vec{v}_1 \frac{1}{\vec{S}_2} \cdot \vec{v}_1 \vec{S}_1 \cdot \vec{v}_2 + \frac{3}{2} \hat{n} \cdot \vec{v}_1 \vec{S}_1 \cdot \vec{v}_2 \vec{S}_2 \cdot \vec{a}_1 - 2 \hat{n} \cdot \vec{v}_2 \vec{S}_1 \cdot \vec{v}_2 \vec{S}_2 \cdot \vec{a}_1 + 5 \hat{n} \cdot \vec{v}_1 \frac{1}{\vec{S}_1} \cdot \vec{v}_2 \vec{S}_2 \cdot \vec{v}_1 - \\ 2 \hat{n} \cdot \vec{v}_2 \frac{1}{\vec{S}_1} \cdot \vec{v}_2 \vec{S}_2 \cdot \vec{v}_1 - 3 \hat{n} \cdot \vec{v}_1 \vec{S}_1 \cdot \vec{a}_2 \vec{S}_2 \cdot \vec{v}_1 + \frac{7}{2} \hat{n} \cdot \vec{a}_1 \vec{S}_1 \cdot \vec{v}_2 \vec{S}_2 \cdot \vec{v}_1 + 3 \hat{n} \cdot \vec{v}_1 \vec{S}_1 \cdot \vec{S}_2 \vec{v}_1 \cdot \vec{a}_2 - \\ 5 \hat{n} \cdot \vec{v}_1 \frac{1}{\vec{S}_1} \cdot \vec{S}_2 \vec{v}_1 \cdot \vec{v}_2 + 2 \hat{n} \cdot \vec{v}_2 \frac{1}{\vec{S}_1} \cdot \vec{S}_2 \vec{v}_1 \cdot \vec{v}_2 + 3 \hat{n} \cdot \vec{v}_1 \vec{S}_1 \cdot \frac{1}{\vec{S}_2} \vec{v}_1 \cdot \vec{v}_2 - \frac{7}{2} \hat{n} \cdot \vec{a}_1 \vec{S}_1 \cdot \vec{S}_2 \vec{v}_1 \cdot \vec{v}_2 \Big) + \\ \frac{1}{r^4} \left( 42 \hat{n} \times \vec{S}_1 \cdot \vec{v}_1 \hat{n} \times \vec{S}_2 \cdot \vec{v}_2 (\hat{n} \cdot \vec{v}_1)^2 + 7 \vec{S}_1 \cdot \vec{v}_2 \vec{S}_2 \cdot \vec{v}_1 (\hat{n} \cdot \vec{v}_1)^2 - 7 \vec{S}_1 \cdot \vec{S}_2 \vec{v}_1 \cdot \vec{v}_2 (\hat{n} \cdot \vec{v}_1)^2 + \right. \\ 12 \hat{n} \times \vec{S}_2 \cdot \vec{v}_2 \vec{S}_1 \times \vec{v}_1 \cdot \vec{v}_2 \hat{n} \cdot \vec{v}_1 + 14 \hat{n} \times \vec{S}_1 \cdot \vec{v}_1 \vec{S}_2 \times \vec{v}_1 \cdot \vec{v}_2 \hat{n} \cdot \vec{v}_1 - 72 \hat{n} \times \vec{S}_1 \cdot \vec{v}_1 \hat{n} \times \vec{S}_2 \cdot \vec{v}_2 \hat{n} \cdot \vec{v}_2 \hat{n} \cdot \vec{v}_1 - \\ 12 \hat{n} \cdot \vec{v}_2 \vec{S}_1 \cdot \vec{v}_2 \vec{S}_2 \cdot \vec{v}_1 \hat{n} \cdot \vec{v}_1 + 12 \hat{n} \cdot \vec{v}_2 \vec{S}_1 \cdot \vec{S}_2 \vec{v}_1 \cdot \vec{v}_2 \hat{n} \cdot \vec{v}_1 - 3 \vec{S}_1 \cdot \vec{S}_2 (\vec{v}_1 \cdot \vec{v}_2)^2 + \\ 3 \vec{S}_1 \times \vec{v}_1 \cdot \vec{v}_2 \vec{S}_2 \times \vec{v}_1 \cdot \vec{v}_2 - 12 \hat{n} \times \vec{S}_1 \cdot \vec{v}_1 \vec{S}_2 \times \vec{v}_1 \cdot \vec{v}_2 \hat{n} \cdot \vec{v}_2 - 4 \hat{n} \times \vec{S}_1 \cdot \vec{v}_1 \hat{n} \times \vec{S}_2 \cdot \vec{v}_2 \vec{v}_1 \cdot \vec{v}_1 - \\ \left. \vec{S}_1 \cdot \vec{v}_2 \vec{S}_2 \cdot \vec{v}_1 \vec{v}_1 \cdot \vec{v}_1 + 12 \hat{n} \times \vec{S}_1 \cdot \vec{v}_1 \hat{n} \times \vec{S}_2 \cdot \vec{v}_2 \vec{v}_1 \cdot \vec{v}_2 + 3 \vec{S}_1 \cdot \vec{v}_2 \vec{S}_2 \cdot \vec{v}_1 \vec{v}_1 \cdot \vec{v}_2 + \vec{S}_1 \cdot \vec{S}_2 \vec{v}_1 \cdot \vec{v}_1 \vec{v}_1 \cdot \vec{v}_2 \right) \Big\} m_1 \Big\}$$

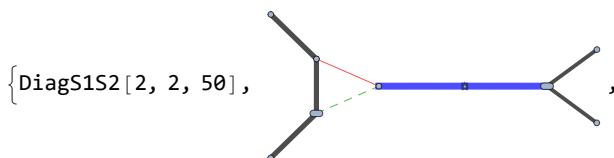

$$\begin{aligned} G^2 \left( \frac{1}{r} \left( \frac{1}{3} \hat{n} \cdot \vec{S}_1 \hat{n} \cdot \vec{a}_2 \hat{n} \cdot \vec{S}_2 - \frac{1}{6} \vec{S}_1 \cdot \vec{a}_2 \hat{n} \cdot \vec{S}_2 + \frac{1}{3} \hat{n} \cdot \vec{S}_1 \hat{n} \cdot \vec{S}_2 \hat{n} \cdot \vec{v}_2 + \right. \right. \\ \left. \frac{1}{3} \hat{n} \cdot \vec{v}_2 \vec{S}_1^2 \cdot \vec{S}_2 + \frac{1}{3} \hat{n} \cdot \vec{a}_2 \vec{S}_1^2 \cdot \vec{S}_2 - \frac{1}{6} \hat{n} \cdot \vec{S}_2 \vec{S}_1^2 \cdot \vec{v}_2 - \frac{1}{6} \hat{n} \cdot \vec{S}_1 \vec{S}_2^2 \cdot \vec{v}_2 - \frac{1}{6} \hat{n} \cdot \vec{S}_1 \vec{S}_2^2 \cdot \vec{a}_2 \right) + \frac{1}{r^2} \\ \left( \frac{4}{3} \hat{n} \cdot \vec{S}_1 \hat{n} \cdot \vec{S}_2 (\hat{n} \cdot \vec{v}_2)^2 + \frac{2}{3} \vec{S}_1^2 \cdot \vec{S}_2 (\hat{n} \cdot \vec{v}_2)^2 - \frac{4}{3} \hat{n} \cdot \vec{S}_1 \hat{n} \cdot \vec{S}_2 \hat{n} \cdot \vec{v}_1 \hat{n} \cdot \vec{v}_2 + \frac{1}{3} \hat{n} \cdot \vec{v}_1 \vec{S}_1^2 \cdot \vec{S}_2 \hat{n} \cdot \vec{v}_2 + \right. \\ \frac{1}{3} \hat{n} \cdot \vec{S}_2 \vec{S}_1^2 \cdot \vec{v}_1 \hat{n} \cdot \vec{v}_2 - \frac{2}{3} \hat{n} \cdot \vec{S}_2 \vec{S}_1^2 \cdot \vec{v}_2 \hat{n} \cdot \vec{v}_2 - \hat{n} \cdot \vec{S}_1 \vec{S}_2^2 \cdot \vec{a}_1 \hat{n} \cdot \vec{v}_2 - \frac{2}{3} \hat{n} \cdot \vec{S}_1 \vec{S}_2^2 \cdot \vec{v}_1 \hat{n} \cdot \vec{v}_2 + \hat{n} \cdot \vec{a}_1 \vec{S}_1^2 \cdot \vec{S}_2 \hat{n} \cdot \vec{v}_2 - \\ \frac{2}{3} \hat{n} \cdot \vec{S}_1 \vec{S}_2^2 \cdot \vec{v}_2 \hat{n} \cdot \vec{v}_2 - \frac{4}{3} \hat{n} \cdot \vec{S}_1 \hat{n} \cdot \vec{a}_2 \hat{n} \cdot \vec{S}_2 \hat{n} \cdot \vec{v}_1 + \frac{1}{3} \hat{n} \cdot \vec{S}_2 \hat{n} \cdot \vec{v}_1 \vec{S}_1^2 \cdot \vec{a}_2 + \frac{1}{3} \hat{n} \cdot \vec{a}_2 \hat{n} \cdot \vec{v}_1 \vec{S}_1^2 \cdot \vec{S}_2 + \\ \frac{1}{3} \hat{n} \cdot \vec{a}_2 \hat{n} \cdot \vec{S}_2 \vec{S}_1^2 \cdot \vec{v}_1 + \frac{1}{3} \hat{n} \cdot \vec{S}_2 \hat{n} \cdot \vec{v}_1 \vec{S}_1^2 \cdot \vec{v}_2 + \frac{1}{3} \vec{S}_1^2 \cdot \vec{v}_2 \vec{S}_2^2 \cdot \vec{v}_1 + \frac{1}{3} \hat{n} \cdot \vec{S}_1 \hat{n} \cdot \vec{v}_1 \vec{S}_2^2 \cdot \vec{v}_2 - \\ \frac{1}{6} \vec{S}_1^2 \cdot \vec{v}_1 \vec{S}_2^2 \cdot \vec{v}_2 - \frac{1}{2} \vec{a}_1 \cdot \vec{v}_2 \vec{S}_1^2 \cdot \vec{S}_2 + \hat{n} \cdot \vec{a}_1 \hat{n} \cdot \vec{a}_2 \vec{S}_1^2 \cdot \vec{S}_2 - \frac{1}{2} \vec{a}_1 \cdot \vec{a}_2 \vec{S}_1^2 \cdot \vec{S}_2 + \frac{1}{2} \vec{S}_2^2 \cdot \vec{a}_1 \vec{S}_1^2 \cdot \vec{v}_2 - \\ \hat{n} \cdot \vec{a}_2 \hat{n} \cdot \vec{S}_1 \vec{S}_2^2 \cdot \vec{a}_1 + \frac{1}{2} \vec{S}_1^2 \cdot \vec{a}_2 \vec{S}_2^2 \cdot \vec{a}_1 + \frac{1}{3} \hat{n} \cdot \vec{S}_1 \hat{n} \cdot \vec{v}_1 \vec{S}_2^2 \cdot \vec{a}_2 - \frac{1}{6} \vec{S}_1^2 \cdot \vec{v}_1 \vec{S}_2^2 \cdot \vec{a}_2 - \\ \left. \frac{2}{3} \hat{n} \cdot \vec{S}_1 \hat{n} \cdot \vec{a}_2 \vec{S}_2^2 \cdot \vec{v}_1 + \frac{1}{3} \vec{S}_1^2 \cdot \vec{a}_2 \vec{S}_2^2 \cdot \vec{v}_1 + \frac{1}{3} \vec{S}_1^2 \cdot \vec{v}_2 \vec{S}_2^2 \cdot \vec{v}_2 + \frac{1}{3} \hat{n} \cdot \vec{S}_1 \hat{n} \cdot \vec{S}_2 \vec{v}_1 \cdot \vec{a}_2 - \frac{1}{6} \vec{S}_1^2 \cdot \vec{S}_2 \vec{v}_1 \cdot \vec{a}_2 + \right. \end{aligned}$$

$\{\text{DiagS1S2}[2, 2, 51],$

$$\begin{aligned} G^2 \left( \frac{1}{r} \left( \frac{2}{3} \hat{n} \cdot \vec{S}_2 \hat{n} \cdot \vec{a}_1 \hat{n} \cdot \vec{S}_1 + \frac{2}{3} \vec{S}_2 \cdot \vec{a}_1 \hat{n} \cdot \vec{S}_1 + \frac{2}{3} \hat{n} \cdot \vec{S}_1 \hat{n} \cdot \vec{S}_2 \hat{n} \cdot \vec{v}_1 - \right. \right. \\ \left. \frac{1}{3} \hat{n} \cdot \vec{v}_1 \vec{S}_1 \cdot \vec{S}_2 - \frac{1}{3} \hat{n} \cdot \vec{S}_2 \vec{S}_1 \cdot \vec{v}_1 + \frac{2}{3} \hat{n} \cdot \vec{S}_1 \vec{S}_2 \cdot \vec{v}_1 - \frac{1}{3} \hat{n} \cdot \vec{a}_1 \vec{S}_1 \cdot \vec{S}_2 - \frac{1}{3} \hat{n} \cdot \vec{S}_2 \vec{S}_1 \cdot \vec{a}_1 \right) + \frac{1}{r^2} \\ \left( -\frac{8}{3} \hat{n} \cdot \vec{S}_1 \hat{n} \cdot \vec{S}_2 (\hat{n} \cdot \vec{a}_1)^2 + \frac{2}{3} \vec{S}_1 \cdot \vec{S}_2 (\hat{n} \cdot \vec{a}_1)^2 + \frac{8}{3} \hat{n} \cdot \vec{a}_2 \hat{n} \cdot \vec{S}_1 \hat{n} \cdot \vec{S}_2 \hat{n} \cdot \vec{a}_1 - \frac{14}{3} \hat{n} \cdot \vec{S}_2 \hat{n} \cdot \vec{S}_1 \hat{n} \cdot \vec{v}_1 \hat{n} \cdot \vec{a}_1 - \right. \\ \frac{8}{3} \hat{n} \cdot \vec{S}_1 \hat{n} \cdot \vec{S}_2 \hat{n} \cdot \vec{v}_1 \hat{n} \cdot \vec{a}_1 + \frac{16}{3} \hat{n} \cdot \vec{S}_2 \hat{n} \cdot \vec{S}_1 \hat{n} \cdot \vec{v}_2 \hat{n} \cdot \vec{a}_1 + \frac{2}{3} \hat{n} \cdot \vec{v}_1 \vec{S}_1 \cdot \vec{S}_2 \hat{n} \cdot \vec{a}_1 + \frac{2}{3} \hat{n} \cdot \vec{S}_2 \vec{S}_1 \cdot \vec{v}_1 \hat{n} \cdot \vec{a}_1 - \\ \frac{7}{3} \hat{n} \cdot \vec{S}_1 \vec{S}_2 \cdot \vec{v}_1 \hat{n} \cdot \vec{a}_1 - \frac{4}{3} \hat{n} \cdot \vec{S}_1 \vec{S}_2 \cdot \vec{v}_2 \hat{n} \cdot \vec{a}_1 + \frac{8}{3} \hat{n} \cdot \vec{v}_1 \vec{S}_1 \cdot \vec{S}_2 \hat{n} \cdot \vec{a}_1 - \frac{4}{3} \hat{n} \cdot \vec{v}_2 \vec{S}_1 \cdot \vec{S}_2 \hat{n} \cdot \vec{a}_1 + \frac{4}{3} \hat{n} \cdot \vec{S}_2 \vec{S}_1 \cdot \vec{a}_1 \hat{n} \cdot \vec{a}_1 - \\ \frac{2}{3} \hat{n} \cdot \vec{S}_2 \vec{S}_1 \cdot \vec{a}_2 \hat{n} \cdot \vec{a}_1 - \frac{2}{3} \hat{n} \cdot \vec{a}_2 \vec{S}_1 \cdot \vec{S}_2 \hat{n} \cdot \vec{a}_1 + \frac{7}{6} \hat{n} \cdot \vec{S}_2 \vec{S}_1 \cdot \vec{v}_1 \hat{n} \cdot \vec{a}_1 - \frac{4}{3} \hat{n} \cdot \vec{S}_2 \vec{S}_1 \cdot \vec{v}_2 \hat{n} \cdot \vec{a}_1 - \frac{2}{3} \hat{n} \cdot \vec{S}_1 \vec{S}_2 \cdot \vec{a}_1 \hat{n} \cdot \vec{a}_1 - \\ \frac{2}{3} \hat{n} \cdot \vec{S}_1 \vec{S}_2 \cdot \vec{a}_2 \hat{n} \cdot \vec{a}_1 + \frac{2}{3} \hat{n} \cdot \vec{S}_1 \vec{S}_2 \cdot \vec{v}_1 \hat{n} \cdot \vec{a}_1 - \frac{14}{3} \hat{n} \cdot \vec{S}_1 \hat{n} \cdot \vec{S}_2 (\hat{n} \cdot \vec{v}_1)^2 - \frac{2}{3} \hat{n} \cdot \vec{S}_2 \hat{n} \cdot \vec{S}_1 (\hat{n} \cdot \vec{v}_1)^2 - \\ 4 \hat{n} \times \vec{S}_1 \cdot \vec{v}_1 \hat{n} \times \vec{S}_2 \cdot \vec{v}_1 - 4 \hat{n} \times \vec{S}_2 \cdot \vec{a}_1 \hat{n} \times \vec{S}_1 \cdot \vec{v}_1 + 2 \hat{n} \times \vec{S}_2 \cdot \vec{v}_1 \hat{n} \times \vec{S}_1 \cdot \vec{v}_1 - 2 \hat{n} \times \vec{S}_1 \cdot \vec{a}_1 \hat{n} \times \vec{S}_2 \cdot \vec{a}_1 - \\ 2 \hat{n} \times \vec{S}_1 \cdot \vec{a}_1 \hat{n} \times \vec{S}_2 \cdot \vec{v}_1 + \frac{8}{3} \hat{n} \cdot \vec{S}_1 \hat{n} \cdot \vec{a}_2 \hat{n} \cdot \vec{S}_2 \hat{n} \cdot \vec{v}_1 + \frac{16}{3} \hat{n} \cdot \vec{S}_1 \hat{n} \cdot \vec{S}_2 \hat{n} \cdot \vec{v}_1 \hat{n} \cdot \vec{v}_2 + \frac{8}{3} (\hat{n} \cdot \vec{v}_1)^2 \vec{S}_1 \cdot \vec{S}_2 - \\ \left. \frac{4}{3} \hat{n} \cdot \vec{v}_1 \hat{n} \cdot \vec{v}_2 \vec{S}_1 \cdot \vec{S}_2 + \frac{2}{3} \hat{n} \cdot \vec{S}_2 \hat{n} \cdot \vec{v}_1 \vec{S}_1 \cdot \vec{a}_1 - \frac{2}{3} \hat{n} \cdot \vec{S}_2 \hat{n} \cdot \vec{v}_1 \vec{S}_1 \cdot \vec{a}_2 - \frac{2}{3} \hat{n} \cdot \vec{a}_2 \hat{n} \cdot \vec{v}_1 \vec{S}_1 \cdot \vec{S}_2 - \frac{2}{3} \hat{n} \cdot \vec{a}_2 \hat{n} \cdot \vec{S}_2 \vec{S}_1 \cdot \vec{v}_1 + \right. \end{aligned}$$





[illegible]

[illegible]

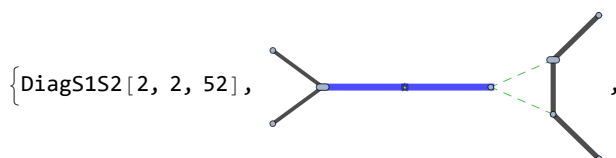

$$\begin{aligned} G^2 \bigg( & \frac{1}{r^2} \left( - \left( \hat{n} \times \vec{S}_1 \cdot \vec{v}_2 \right) \hat{n} \times \vec{S}_2 \cdot \vec{v}_1 + \hat{n} \times \vec{S}_1 \cdot \vec{v}_1 \hat{n} \times \vec{S}_2 \cdot \vec{v}_2 + \hat{n} \times \vec{S}_2 \cdot \vec{v}_2 \hat{n} \times \vec{S}_1 \cdot \vec{a}_1 - \hat{n} \times \vec{S}_2 \cdot \vec{a}_1 \hat{n} \times \vec{S}_1 \cdot \vec{v}_2 - \right. \\ & \hat{n} \times \vec{S}_1 \cdot \vec{a}_2 \hat{n} \times \vec{S}_2 \cdot \vec{a}_1 + \hat{n} \times \vec{S}_1 \cdot \vec{v}_1 \hat{n} \times \vec{S}_2 \cdot \vec{a}_2 + \hat{n} \times \vec{S}_1 \cdot \vec{a}_1 \hat{n} \times \vec{S}_2 \cdot \vec{a}_2 - \hat{n} \times \vec{S}_1 \cdot \vec{a}_2 \hat{n} \times \vec{S}_2 \cdot \vec{v}_1 - \\ & \hat{n} \cdot \vec{v}_1 \hat{n} \cdot \vec{v}_2 \vec{S}_1 \cdot \vec{S}_2 - \hat{n} \cdot \vec{a}_2 \hat{n} \cdot \vec{v}_1 \vec{S}_1 \cdot \vec{S}_2 + \hat{n} \cdot \vec{S}_1 \hat{n} \cdot \vec{v}_2 \vec{S}_2 \cdot \vec{a}_1 + \hat{n} \cdot \vec{S}_1 \hat{n} \cdot \vec{v}_2 \vec{S}_2 \cdot \vec{v}_1 - \frac{1}{2} \vec{S}_1 \cdot \vec{v}_1 \vec{S}_2 \cdot \vec{v}_2 + \\ & \hat{n} \cdot \vec{S}_1 \hat{n} \cdot \vec{S}_2 \vec{a}_1 \cdot \vec{a}_2 + \hat{n} \cdot \vec{S}_2 \hat{n} \cdot \vec{S}_1 \vec{a}_1 \cdot \vec{v}_2 - \hat{n} \cdot \vec{a}_1 \hat{n} \cdot \vec{v}_2 \vec{S}_1 \cdot \vec{S}_2 + \frac{1}{2} \vec{a}_1 \cdot \vec{v}_2 \vec{S}_1 \cdot \vec{S}_2 - \frac{1}{2} \vec{S}_2 \cdot \vec{v}_2 \vec{S}_1 \cdot \vec{a}_1 - \\ & \hat{n} \cdot \vec{a}_1 \hat{n} \cdot \vec{a}_2 \vec{S}_1 \cdot \vec{S}_2 + \frac{1}{2} \vec{a}_1 \cdot \vec{a}_2 \vec{S}_1 \cdot \vec{S}_2 + \hat{n} \cdot \vec{a}_2 \hat{n} \cdot \vec{S}_1 \vec{S}_2 \cdot \vec{a}_1 - \frac{1}{2} \vec{S}_1 \cdot \vec{v}_1 \vec{S}_2 \cdot \vec{a}_2 - \frac{1}{2} \vec{S}_1 \cdot \vec{a}_1 \vec{S}_2 \cdot \vec{a}_2 + \\ & \left. \hat{n} \cdot \vec{S}_1 \hat{n} \cdot \vec{a}_2 \vec{S}_2 \cdot \vec{v}_1 + \hat{n} \cdot \vec{S}_1 \hat{n} \cdot \vec{S}_2 \vec{v}_1 \cdot \vec{a}_2 + \frac{1}{2} \vec{S}_1 \cdot \vec{S}_2 \vec{v}_1 \cdot \vec{a}_2 + \hat{n} \cdot \vec{S}_1 \hat{n} \cdot \vec{S}_2 \vec{v}_1 \cdot \vec{v}_2 + \frac{1}{2} \vec{S}_1 \cdot \vec{S}_2 \vec{v}_1 \cdot \vec{v}_2 \right) + \frac{1}{r^3} \end{aligned}$$

$\{\text{DiagS1S2}[2, 2, 53],$

$$\begin{aligned} G^2 & \left( \frac{1}{r^2} \left( 2 \vec{S}_1 \cdot \vec{S}_2 \left( \hat{n} \cdot \vec{a}_1 \right)^2 + 2 \hat{n} \cdot \vec{v}_1 \vec{S}_1 \cdot \vec{S}_2 \hat{n} \cdot \vec{a}_1 + 4 \hat{n} \cdot \vec{S}_1 \vec{S}_2 \cdot \vec{v}_1 \hat{n} \cdot \vec{a}_1 + 2 \hat{n} \cdot \vec{v}_1 \vec{S}_1 \cdot \vec{S}_2 \hat{n} \cdot \vec{a}_1 - 2 \hat{n} \cdot \vec{S}_1 \vec{S}_2 \cdot \vec{a}_1 \hat{n} \cdot \vec{a}_1 - \right. \right. \\ & 6 \hat{n} \cdot \vec{S}_1 \vec{S}_2 \cdot \vec{v}_1 \hat{n} \cdot \vec{a}_1 + 4 \hat{n} \times \vec{S}_1 \cdot \vec{v}_1 \hat{n} \times \vec{S}_2 \cdot \vec{v}_1 + 2 \hat{n} \times \vec{S}_2 \cdot \vec{v}_1 \hat{n} \times \vec{S}_1 \cdot \vec{a}_1 + 2 \hat{n} \times \vec{S}_2 \cdot \vec{a}_1 \hat{n} \times \vec{S}_1 \cdot \vec{v}_1 + \\ & 2 \hat{n} \times \vec{S}_1 \cdot \vec{v}_1 \hat{n} \times \vec{S}_2 \cdot \vec{a}_1 + 4 \hat{n} \times \vec{S}_1 \cdot \vec{a}_1 \hat{n} \times \vec{S}_2 \cdot \vec{a}_1 + 2 \hat{n} \times \vec{S}_1 \cdot \vec{a}_1 \hat{n} \times \vec{S}_2 \cdot \vec{v}_1 + 2 \left( \hat{n} \cdot \vec{v}_1 \right)^2 \vec{S}_1 \cdot \vec{S}_2 - 6 \hat{n} \cdot \vec{S}_1 \hat{n} \cdot \vec{v}_1 \vec{S}_2 \cdot \vec{a}_1 - \\ & 2 \hat{n} \cdot \vec{S}_1 \hat{n} \cdot \vec{v}_1 \vec{S}_2 \cdot \vec{v}_1 + 3 \vec{S}_1 \cdot \vec{v}_1 \vec{S}_2 \cdot \vec{v}_1 + 2 \hat{n} \cdot \vec{S}_1 \hat{n} \cdot \vec{S}_2 \vec{a}_1 \cdot \vec{a}_1 - \vec{S}_2 \cdot \vec{v}_1 \vec{S}_1 \cdot \vec{a}_1 - 3 \vec{a}_1 \cdot \vec{a}_1 \vec{S}_1 \cdot \vec{S}_2 + 4 \vec{S}_2 \cdot \vec{a}_1 \vec{S}_1 \cdot \vec{v}_1 + \\ & 4 \hat{n} \cdot \vec{S}_1 \hat{n} \cdot \vec{v}_1 \vec{S}_2 \cdot \vec{a}_1 - \vec{S}_1 \cdot \vec{v}_1 \vec{S}_2 \cdot \vec{a}_1 + 3 \vec{S}_1 \cdot \vec{a}_1 \vec{S}_2 \cdot \vec{a}_1 + 4 \vec{S}_1 \cdot \vec{a}_1 \vec{S}_2 \cdot \vec{v}_1 + 2 \hat{n} \cdot \vec{S}_2 \hat{n} \cdot \vec{S}_1 \vec{v}_1 \cdot \vec{a}_1 + \\ & \left. 2 \hat{n} \cdot \vec{S}_1 \hat{n} \cdot \vec{S}_2 \vec{v}_1 \cdot \vec{a}_1 - 3 \vec{S}_1 \cdot \vec{S}_2 \vec{v}_1 \cdot \vec{a}_1 - 3 \vec{S}_1 \cdot \vec{S}_2 \vec{v}_1 \cdot \vec{a}_1 + 2 \hat{n} \cdot \vec{S}_1 \hat{n} \cdot \vec{S}_2 \vec{v}_1 \cdot \vec{v}_1 - 3 \vec{S}_1 \cdot \vec{S}_2 \vec{v}_1 \cdot \vec{v}_1 \right) + \\ & \frac{1}{r^3} \left( -6 \vec{S}_1 \cdot \vec{S}_2 \left( \hat{n} \cdot \vec{v}_1 \right)^3 - 2 \vec{S}_1 \cdot \vec{S}_2 \left( \hat{n} \cdot \vec{v}_1 \right)^3 + 8 \hat{n} \cdot \vec{v}_2 \vec{S}_1 \cdot \vec{S}_2 \left( \hat{n} \cdot \vec{v}_1 \right)^2 + 2 \hat{n} \cdot \vec{S}_1 \vec{S}_2 \cdot \vec{v}_1 \left( \hat{n} \cdot \vec{v}_1 \right)^2 - \right. \\ & \left. 8 \hat{n} \cdot \vec{a}_1 \vec{S}_1 \cdot \vec{S}_2 \left( \hat{n} \cdot \vec{v}_1 \right)^2 + 14 \hat{n} \cdot \vec{S}_1 \vec{S}_2 \cdot \vec{a}_1 \left( \hat{n} \cdot \vec{v}_1 \right)^2 + 6 \hat{n} \cdot \vec{S}_1 \vec{S}_2 \cdot \vec{v}_1 \left( \hat{n} \cdot \vec{v}_1 \right)^2 + 8 \hat{n} \times \vec{S}_2 \cdot \vec{v}_1 \hat{n} \times \vec{S}_1 \cdot \vec{v}_1 \hat{n} \cdot \vec{v}_1 + \right. \end{aligned}$$

[illegible]

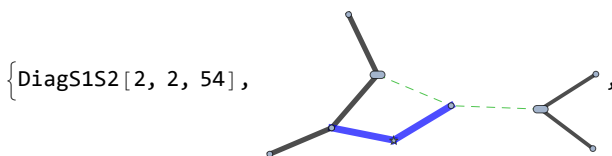

$$\begin{aligned} G^2 & \left( \frac{1}{r^2} \left( -2 \hat{n} \times \vec{S_2} \cdot \vec{v_1} \hat{n} \times \vec{S_1} \cdot \vec{a_1} - 2 \hat{n} \times \vec{S_2} \cdot \vec{a_1} \hat{n} \times \vec{S_1} \cdot \vec{v_1} - 2 \hat{n} \times \vec{S_1} \cdot \vec{v_1} \hat{n} \times \vec{S_2} \cdot \vec{a_1} - \right. \right. \\ & 2 \hat{n} \times \vec{S_1} \cdot \vec{a_1} \hat{n} \times \vec{S_2} \cdot \vec{v_1} - 16 \hat{n} \cdot \vec{S_2} \hat{n} \cdot \vec{a_1} \hat{n} \cdot \vec{S_1} \hat{n} \cdot \vec{v_1} - 16 \hat{n} \cdot \vec{S_1} \hat{n} \cdot \vec{a_1} \hat{n} \cdot \vec{S_2} \hat{n} \cdot \vec{v_1} + 4 \hat{n} \cdot \vec{S_2} \hat{n} \cdot \vec{v_1} \vec{S_1} \cdot \vec{a_1} + \\ & 4 \hat{n} \cdot \vec{a_1} \hat{n} \cdot \vec{S_2} \vec{S_1} \cdot \vec{v_1} + 4 \hat{n} \cdot \vec{S_2} \hat{n} \cdot \vec{v_1} \vec{S_1} \cdot \vec{a_1} - \vec{S_2} \cdot \vec{v_1} \vec{S_1} \cdot \vec{a_1} + 4 \hat{n} \cdot \vec{S_2} \hat{n} \cdot \vec{a_1} \vec{S_1} \cdot \vec{v_1} - \\ & \left. \vec{S_2} \cdot \vec{a_1} \vec{S_1} \cdot \vec{v_1} - \vec{S_1} \cdot \vec{v_1} \vec{S_2} \cdot \vec{a_1} - \vec{S_1} \cdot \vec{a_1} \vec{S_2} \cdot \vec{v_1} + 2 \vec{S_1} \cdot \vec{S_2} \vec{v_1} \cdot \vec{a_1} + 2 \vec{S_1} \cdot \vec{S_2} \vec{v_1} \cdot \vec{a_1} \right) + \frac{1}{r^3} \\ & \left( -12 \hat{n} \cdot \vec{S_2} \hat{n} \cdot \vec{S_1} (\hat{n} \cdot \vec{v_1})^3 - 12 \hat{n} \cdot \vec{S_1} \hat{n} \cdot \vec{S_2} (\hat{n} \cdot \vec{v_1})^3 - 2 \vec{S_1} \cdot \vec{S_2} (\hat{n} \cdot \vec{v_1})^3 - 2 \vec{S_1} \cdot \vec{S_2} (\hat{n} \cdot \vec{v_1})^3 + \right. \\ & \left. 120 \hat{n} \cdot \vec{a_1} \hat{n} \cdot \vec{S_1} \hat{n} \cdot \vec{S_2} (\hat{n} \cdot \vec{v_1})^2 + 6 \hat{n} \cdot \vec{S_2} \vec{S_1} \cdot \vec{v_1} (\hat{n} \cdot \vec{v_1})^2 + 4 \hat{n} \cdot \vec{S_1} \vec{S_2} \cdot \vec{v_1} (\hat{n} \cdot \vec{v_1})^2 - \right. \end{aligned}$$

$$\{\text{DiagS1S2}[2, 2, 55],$$

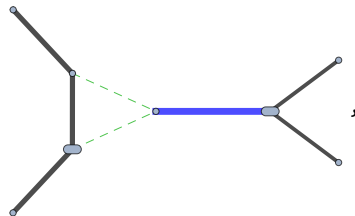

$$G^2 \left( \frac{-4 \hat{n} \times \vec{S}_1 \cdot \vec{v}_2 \hat{n} \times \vec{S}_2 \cdot \vec{a}_1 + 4 \hat{n} \cdot \vec{S}_1 \hat{n} \cdot \vec{S}_2 \vec{a}_1 \cdot \vec{v}_2 + 2 \vec{S}_1 \cdot \vec{S}_2 \vec{a}_1 \cdot \vec{v}_2 - 2 \vec{S}_1 \cdot \vec{a}_1 \vec{S}_2 \cdot \vec{v}_2}{r^2} + \frac{1}{r^3} \right.$$
$$\left. \begin{aligned} & \left( 10 \hat{n} \times \vec{S}_2 \cdot \vec{v}_1 \vec{S}_1 \times \vec{v}_1 \cdot \vec{v}_2 + \frac{3}{2} \hat{n} \times \vec{S}_1 \cdot \vec{v}_2 \vec{S}_2 \times \vec{v}_1 \cdot \vec{v}_2 + 8 \hat{n} \times \vec{S}_2 \cdot \vec{v}_1 \vec{S}_1 \times \vec{a}_1 \cdot \vec{v}_2 + 12 \hat{n} \times \vec{S}_2 \cdot \vec{v}_2 \vec{S}_1 \times \vec{v}_1 \cdot \vec{a}_1 + \right. \\ & 2 \hat{n} \times \vec{S}_2 \cdot \vec{a}_1 \vec{S}_1 \times \vec{v}_1 \cdot \vec{v}_2 + 3 \hat{n} \times \vec{S}_1 \cdot \vec{v}_2 \vec{S}_2 \times \vec{v}_1 \cdot \vec{a}_1 + 2 \hat{n} \times \vec{S}_1 \cdot \vec{v}_2 \vec{S}_2 \times \vec{v}_1 \cdot \vec{a}_2 + \hat{n} \times \vec{S}_1 \cdot \vec{a}_2 \vec{S}_2 \times \vec{v}_1 \cdot \vec{v}_2 + \\ & 4 \hat{n} \times \vec{S}_1 \cdot \vec{v}_1 \hat{n} \times \vec{S}_2 \cdot \vec{v}_2 \hat{n} \cdot \vec{a}_2 + 12 \hat{n} \times \vec{S}_1 \cdot \vec{v}_2 \hat{n} \times \vec{S}_2 \cdot \vec{a}_1 \hat{n} \cdot \vec{v}_1 + 4 \hat{n} \times \vec{S}_1 \cdot \vec{v}_2 \hat{n} \times \vec{S}_2 \cdot \vec{v}_1 \hat{n} \cdot \vec{v}_1 + \\ & \left. 6 \hat{n} \times \vec{S}_2 \cdot \vec{v}_2 \hat{n} \times \vec{S}_1 \cdot \vec{v}_1 \hat{n} \cdot \vec{v}_2 + 8 \hat{n} \times \vec{S}_1 \cdot \vec{v}_1 \hat{n} \times \vec{S}_2 \cdot \vec{a}_2 \hat{n} \cdot \vec{v}_2 - 12 \hat{n} \cdot \vec{S}_1 \hat{n} \cdot \vec{S}_2 \hat{n} \cdot \vec{v}_1 \vec{a}_1 \cdot \vec{v}_2 - 2 \hat{n} \cdot \vec{v}_1 \vec{a}_1 \cdot \vec{v}_2 \vec{S}_1 \cdot \vec{S}_2 + \right. \end{aligned}$$



$$\left. \begin{aligned} & 8 \hat{n} \times \vec{S}_1 \cdot \vec{v}_1 \vec{S}_2 \times \vec{v}_1 \cdot \vec{v}_2 \hat{n} \cdot \vec{v}_2 + 2 \hat{n} \times \vec{S}_1 \cdot \vec{v}_1 \hat{n} \times \vec{S}_2 \cdot \vec{v}_1 \vec{v}_1 \cdot \vec{v}_1 + 18 \hat{n} \times \vec{S}_1 \cdot \vec{v}_2 \hat{n} \times \vec{S}_2 \cdot \vec{v}_2 \vec{v}_1 \cdot \vec{v}_1 - \\ & 6 (\hat{n} \cdot \vec{v}_2)^2 \vec{S}_1 \cdot \vec{S}_2 \vec{v}_1 \cdot \vec{v}_1 + 4 \hat{n} \cdot \vec{S}_2 \hat{n} \cdot \vec{v}_2 \vec{S}_1 \cdot \vec{v}_1 \vec{v}_1 \cdot \vec{v}_1 + 6 \hat{n} \cdot \vec{S}_2 \hat{n} \cdot \vec{v}_2 \vec{S}_1 \cdot \vec{v}_2 \vec{v}_1 \cdot \vec{v}_1 + \\ & 8 \hat{n} \cdot \vec{S}_1 \hat{n} \cdot \vec{v}_2 \vec{S}_2 \cdot \vec{v}_1 \vec{v}_1 \cdot \vec{v}_1 - \vec{S}_1 \cdot \vec{v}_1 \vec{S}_2 \cdot \vec{v}_1 \vec{v}_1 \cdot \vec{v}_1 - 2 \vec{S}_1 \cdot \vec{v}_2 \vec{S}_2 \cdot \vec{v}_1 \vec{v}_1 \cdot \vec{v}_1 - \vec{S}_1 \cdot \vec{v}_1 \vec{S}_2 \cdot \vec{v}_2 \vec{v}_1 \cdot \vec{v}_1 + \\ & 3 \vec{S}_1 \cdot \vec{v}_2 \vec{S}_2 \cdot \vec{v}_2 \vec{v}_1 \cdot \vec{v}_1 - 4 \hat{n} \times \vec{S}_1 \cdot \vec{v}_1 \hat{n} \times \vec{S}_2 \cdot \vec{v}_1 \vec{v}_1 \cdot \vec{v}_2 - 24 \hat{n} \times \vec{S}_1 \cdot \vec{v}_1 \hat{n} \times \vec{S}_2 \cdot \vec{v}_2 \vec{v}_1 \cdot \vec{v}_2 - \vec{S}_1 \cdot \vec{v}_1 \vec{S}_2 \cdot \vec{v}_1 \vec{v}_1 \cdot \vec{v}_2 - \\ & \frac{11}{2} \vec{S}_1 \cdot \vec{v}_2 \vec{S}_2 \cdot \vec{v}_1 \vec{v}_1 \cdot \vec{v}_2 + 4 \hat{n} \cdot \vec{S}_1 \hat{n} \cdot \vec{S}_2 \vec{v}_1 \cdot \vec{v}_1 \vec{v}_1 \cdot \vec{v}_2 + 2 \vec{S}_1 \cdot \vec{S}_2 \vec{v}_1 \cdot \vec{v}_1 \vec{v}_1 \cdot \vec{v}_2 - 3 \vec{S}_1 \cdot \vec{S}_2 \vec{v}_1 \cdot \vec{v}_1 \vec{v}_2 \cdot \vec{v}_2 \end{aligned} \right) m_1 \}$$

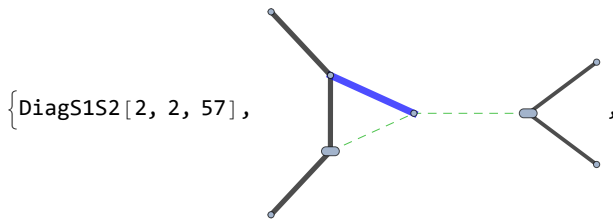

$$G^2 \left( \frac{-4 \hat{n} \times \vec{S_1} \cdot \vec{v_1} \hat{n} \times \vec{S_2} \cdot \vec{v_1} - 2 \vec{S_1} \cdot \vec{v_1} \vec{S_2} \cdot \vec{v_1} + 2 \vec{S_1} \cdot \vec{S_2} \vec{v_1} \cdot \vec{v_1}}{r^2} + \frac{1}{r^3} \right. \\ \left( -32 \vec{S_1} \cdot \vec{S_2} (\hat{n} \cdot \vec{v_1})^3 + 24 \hat{n} \cdot \vec{v_2} \vec{S_1} \cdot \vec{S_2} (\hat{n} \cdot \vec{v_1})^2 - 24 \hat{n} \cdot \vec{S_2} \vec{S_1} \cdot \vec{a_2} (\hat{n} \cdot \vec{v_1})^2 - 32 \hat{n} \cdot \vec{a_1} \vec{S_1} \cdot \vec{S_2} (\hat{n} \cdot \vec{v_1})^2 + \right. \\ 24 \hat{n} \cdot \vec{a_2} \vec{S_1} \cdot \vec{S_2} (\hat{n} \cdot \vec{v_1})^2 - 24 \hat{n} \cdot \vec{S_2} \vec{S_1} \cdot \vec{v_2} (\hat{n} \cdot \vec{v_1})^2 + 32 \hat{n} \cdot \vec{S_1} \vec{S_2} \cdot \vec{a_1} (\hat{n} \cdot \vec{v_1})^2 + \\ 32 \hat{n} \cdot \vec{S_1} \vec{S_2} \cdot \vec{v_1} (\hat{n} \cdot \vec{v_1})^2 + 12 \hat{n} \times \vec{S_2} \cdot \vec{v_1} \hat{n} \times \vec{S_1} \cdot \vec{v_1} \hat{n} \cdot \vec{v_1} + 3 \vec{S_2} \cdot \vec{v_1} \vec{S_1} \cdot \vec{v_1} \hat{n} \cdot \vec{v_1} + 8 \vec{S_2} \cdot \vec{v_1} \vec{S_1} \cdot \vec{v_2} \hat{n} \cdot \vec{v_1} - \\ 16 \vec{S_1} \cdot \vec{v_1} \vec{S_2} \cdot \vec{a_1} \hat{n} \cdot \vec{v_1} - 16 \vec{S_1} \cdot \vec{v_1} \vec{S_2} \cdot \vec{v_1} \hat{n} \cdot \vec{v_1} + 8 \vec{S_1} \cdot \vec{a_2} \vec{S_2} \cdot \vec{v_1} \hat{n} \cdot \vec{v_1} + 16 \vec{S_1} \cdot \vec{S_2} \vec{v_1} \cdot \vec{a_1} \hat{n} \cdot \vec{v_1} - \\ 8 \vec{S_1} \cdot \vec{S_2} \vec{v_1} \cdot \vec{a_2} \hat{n} \cdot \vec{v_1} + 16 \vec{S_1} \cdot \vec{S_2} \vec{v_1} \cdot \vec{v_1} \hat{n} \cdot \vec{v_1} - 3 \vec{S_1} \cdot \vec{S_2} \vec{v_1} \cdot \vec{v_1} \hat{n} \cdot \vec{v_1} - 8 \vec{S_1} \cdot \vec{S_2} \vec{v_1} \cdot \vec{v_2} \hat{n} \cdot \vec{v_1} + \\ 4 \hat{n} \times \vec{S_2} \cdot \vec{v_1} \vec{S_1} \times \vec{v_1} \cdot \vec{v_2} - 2 \hat{n} \times \vec{S_1} \cdot \vec{v_1} \vec{S_2} \times \vec{v_1} \cdot \vec{v_2} + 8 \hat{n} \times \vec{S_2} \cdot \vec{v_1} \vec{S_1} \times \vec{v_1} \cdot \vec{a_1} - 2 \hat{n} \times \vec{S_1} \cdot \vec{v_1} \vec{S_2} \times \vec{v_1} \cdot \vec{a_2} + \\ 4 \hat{n} \times \vec{S_1} \cdot \vec{v_1} \vec{S_2} \times \vec{v_1} \cdot \vec{v_2} - 16 \hat{n} \times \vec{S_1} \cdot \vec{v_1} \hat{n} \times \vec{S_2} \cdot \vec{v_1} \hat{n} \cdot \vec{v_2} - 4 \hat{n} \cdot \vec{v_2} \vec{S_1} \cdot \vec{v_1} \vec{S_2} \cdot \vec{v_1} + 4 \hat{n} \cdot \vec{v_2} \vec{S_1} \cdot \vec{S_2} \vec{v_1} \cdot \vec{v_1} - \\ 4 \hat{n} \cdot \vec{v_2} \vec{S_1} \cdot \vec{S_2} \vec{v_1} \cdot \vec{v_1} + 4 \hat{n} \cdot \vec{S_2} \vec{S_1} \cdot \vec{a_2} \vec{v_1} \cdot \vec{v_1} - 4 \hat{n} \cdot \vec{a_2} \vec{S_1} \cdot \vec{S_2} \vec{v_1} \cdot \vec{v_1} + 4 \hat{n} \cdot \vec{S_2} \vec{S_1} \cdot \vec{v_2} \vec{v_1} \cdot \vec{v_1} \Big) + \\ \left. \frac{1}{r^4} \left( 36 \vec{S_1} \cdot \vec{S_2} (\hat{n} \cdot \vec{v_1})^4 - 36 \hat{n} \cdot \vec{S_1} \vec{S_2} \cdot \vec{v_1} (\hat{n} \cdot \vec{v_1})^3 - 108 \hat{n} \times \vec{S_1} \cdot \vec{v_1} \hat{n} \times \vec{S_2} \cdot \vec{v_1} (\hat{n} \cdot \vec{v_1})^2 - \right. \right. \\ 108 \hat{n} \times \vec{S_1} \cdot \vec{v_2} \hat{n} \times \vec{S_2} \cdot \vec{v_2} (\hat{n} \cdot \vec{v_1})^2 + 36 (\hat{n} \cdot \vec{v_2})^2 \vec{S_1} \cdot \vec{S_2} (\hat{n} \cdot \vec{v_1})^2 - 36 \hat{n} \cdot \vec{S_2} \hat{n} \cdot \vec{v_2} \vec{S_1} \cdot \vec{v_2} (\hat{n} \cdot \vec{v_1})^2 - \\ 12 \vec{S_1} \cdot \vec{v_2} \vec{S_2} \cdot \vec{v_2} (\hat{n} \cdot \vec{v_1})^2 + 36 \hat{n} \cdot \vec{S_1} \hat{n} \cdot \vec{S_2} \vec{v_1} \cdot \vec{v_1} (\hat{n} \cdot \vec{v_1})^2 - 16 \vec{S_1} \cdot \vec{S_2} \vec{v_1} \cdot \vec{v_1} (\hat{n} \cdot \vec{v_1})^2 + \\ 12 \vec{S_1} \cdot \vec{S_2} \vec{v_2} \cdot \vec{v_2} (\hat{n} \cdot \vec{v_1})^2 - 12 \hat{n} \times \vec{S_2} \cdot \vec{v_1} \vec{S_1} \times \vec{v_1} \cdot \vec{v_2} \hat{n} \cdot \vec{v_1} - 24 \hat{n} \times \vec{S_2} \cdot \vec{v_2} \vec{S_1} \times \vec{v_1} \cdot \vec{v_2} \hat{n} \cdot \vec{v_1} - \\ 12 \hat{n} \times \vec{S_1} \cdot \vec{v_1} \vec{S_2} \times \vec{v_1} \cdot \vec{v_2} \hat{n} \cdot \vec{v_1} - 36 \hat{n} \times \vec{S_1} \cdot \vec{v_2} \vec{S_2} \times \vec{v_1} \cdot \vec{v_2} \hat{n} \cdot \vec{v_1} + 72 \hat{n} \times \vec{S_1} \cdot \vec{v_1} \hat{n} \times \vec{S_2} \cdot \vec{v_1} \hat{n} \cdot \vec{v_2} \hat{n} \cdot \vec{v_1} + \\ 12 \hat{n} \cdot \vec{v_2} \vec{S_1} \cdot \vec{v_1} \vec{S_2} \cdot \vec{v_1} \hat{n} \cdot \vec{v_1} + 8 \hat{n} \cdot \vec{v_2} \vec{S_1} \cdot \vec{v_2} \vec{S_2} \cdot \vec{v_1} \hat{n} \cdot \vec{v_1} - 12 \hat{n} \cdot \vec{v_2} \vec{S_1} \cdot \vec{S_2} \vec{v_1} \cdot \vec{v_1} \hat{n} \cdot \vec{v_1} - \\ 12 \hat{n} \cdot \vec{S_2} \vec{S_1} \cdot \vec{v_1} \vec{v_1} \cdot \vec{v_1} \hat{n} \cdot \vec{v_1} + 4 \hat{n} \cdot \vec{S_1} \vec{S_2} \cdot \vec{v_1} \vec{v_1} \cdot \vec{v_1} \hat{n} \cdot \vec{v_1} - 20 \hat{n} \cdot \vec{v_2} \vec{S_1} \cdot \vec{S_2} \vec{v_1} \cdot \vec{v_2} \hat{n} \cdot \vec{v_1} + \\ 12 \hat{n} \cdot \vec{S_2} \vec{S_1} \cdot \vec{v_2} \vec{v_1} \cdot \vec{v_2} \hat{n} \cdot \vec{v_1} - 4 \hat{n} \cdot \vec{S_1} \hat{n} \cdot \vec{S_2} (\vec{v_1} \cdot \vec{v_1})^2 - 2 \vec{S_1} \cdot \vec{S_2} (\vec{v_1} \cdot \vec{v_1})^2 + \frac{1}{2} \vec{S_1} \cdot \vec{S_2} (\vec{v_1} \cdot \vec{v_2})^2 - \\ \frac{11}{2} \vec{S_1} \times \vec{v_1} \cdot \vec{v_2} \vec{S_2} \times \vec{v_1} \cdot \vec{v_2} - 2 \hat{n} \times \vec{S_1} \cdot \vec{v_1} \vec{S_2} \times \vec{v_1} \cdot \vec{v_2} \hat{n} \cdot \vec{v_2} + 20 \hat{n} \times \vec{S_1} \cdot \vec{v_1} \hat{n} \times \vec{S_2} \cdot \vec{v_1} \vec{v_1} \cdot \vec{v_1} + \\ 12 \hat{n} \times \vec{S_1} \cdot \vec{v_2} \hat{n} \times \vec{S_2} \cdot \vec{v_2} \vec{v_1} \cdot \vec{v_1} - 4 (\hat{n} \cdot \vec{v_2})^2 \vec{S_1} \cdot \vec{S_2} \vec{v_1} \cdot \vec{v_1} + 4 \hat{n} \cdot \vec{S_2} \hat{n} \cdot \vec{v_2} \vec{S_1} \cdot \vec{v_2} \vec{v_1} \cdot \vec{v_1} + \\ 4 \vec{S_1} \cdot \vec{v_1} \vec{S_2} \cdot \vec{v_1} \vec{v_1} \cdot \vec{v_1} + 2 \vec{S_1} \cdot \vec{v_2} \vec{S_2} \cdot \vec{v_2} \vec{v_1} \cdot \vec{v_1} - 12 \hat{n} \times \vec{S_1} \cdot \vec{v_1} \hat{n} \times \vec{S_2} \cdot \vec{v_1} \vec{v_1} \cdot \vec{v_2} + 6 \hat{n} \times \vec{S_1} \cdot \vec{v_1} \hat{n} \times \vec{S_2} \cdot \vec{v_2} \vec{v_1} \cdot \vec{v_2} - \\ \left. \left. 3 \vec{S_1} \cdot \vec{v_1} \vec{S_2} \cdot \vec{v_1} \vec{v_1} \cdot \vec{v_2} - \frac{1}{2} \vec{S_1} \cdot \vec{v_2} \vec{S_2} \cdot \vec{v_1} \vec{v_1} \cdot \vec{v_2} + 3 \vec{S_1} \cdot \vec{S_2} \vec{v_1} \cdot \vec{v_1} \vec{v_1} \cdot \vec{v_2} - 2 \vec{S_1} \cdot \vec{S_2} \vec{v_1} \cdot \vec{v_1} \vec{v_2} \cdot \vec{v_2} \right) \right\} m_1 \Bigg) \\ \left. \right\} m_1 \Bigg)$$



$\{\text{DiagS1S2}[2, 2, 58],$

[illegible]

$$\{\text{DiagS1S2}[2, 2, 59],$$

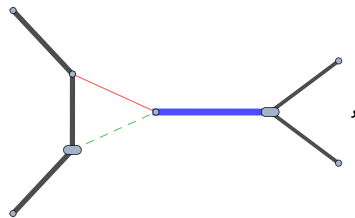

$$G^2 \left( \frac{1}{r^2} \left( \frac{3}{2} \frac{\vec{1}}{S_1} \cdot \vec{S}_2 (\hat{n} \cdot \vec{v}_2)^2 - 2 \hat{n} \cdot \vec{S}_2 \frac{\vec{1}}{S_1} \cdot \vec{a}_2 \hat{n} \cdot \vec{v}_2 - 16 \hat{n} \cdot \vec{a}_1 \frac{\vec{1}}{S_1} \cdot \vec{S}_2 \hat{n} \cdot \vec{v}_2 + 3 \hat{n} \cdot \vec{a}_2 \frac{\vec{1}}{S_1} \cdot \vec{S}_2 \hat{n} \cdot \vec{v}_2 - \frac{3}{2} \hat{n} \cdot \vec{S}_2 \frac{\vec{1}}{S_1} \cdot \vec{v}_2 \hat{n} \cdot \vec{v}_2 - \right. \right.$$

$$\begin{aligned} & 8 \hat{n} \cdot \vec{v}_1 \vec{S}_1 \cdot \vec{S}_2 \hat{n} \cdot \vec{v}_2 - 8 \hat{n} \cdot \vec{a}_1 \vec{S}_1 \cdot \vec{S}_2 \hat{n} \cdot \vec{v}_2 + 8 \hat{n} \cdot \vec{S}_1 \vec{S}_2 \cdot \vec{a}_1 \hat{n} \cdot \vec{v}_2 + 16 \hat{n} \cdot \vec{S}_1 \vec{S}_2 \cdot \vec{a}_1 \hat{n} \cdot \vec{v}_2 + 8 \hat{n} \cdot \vec{S}_1 \vec{S}_2 \cdot \vec{v}_1 \hat{n} \cdot \vec{v}_2 - \\ & \frac{3}{2} \hat{n} \times \vec{S}_1 \cdot \vec{v}_2 \hat{n} \times \vec{S}_2 \cdot \vec{v}_2 - 2 \hat{n} \times \vec{S}_1 \cdot \vec{v}_2 \hat{n} \times \vec{S}_2 \cdot \vec{a}_2 - \hat{n} \times \vec{S}_1 \cdot \vec{a}_2 \hat{n} \times \vec{S}_2 \cdot \vec{v}_2 - \hat{n} \cdot \vec{a}_2 \hat{n} \cdot \vec{S}_2 \vec{S}_1 \cdot \vec{v}_2 + 8 \vec{S}_1 \cdot \vec{S}_2 \vec{a}_1 \cdot \vec{v}_2 + \\ & 4 \vec{a}_1 \cdot \vec{v}_2 \vec{S}_1 \cdot \vec{S}_2 - 4 \vec{S}_1 \cdot \vec{v}_2 \vec{S}_2 \cdot \vec{a}_1 - 8 \vec{S}_1 \cdot \vec{v}_2 \vec{S}_2 \cdot \vec{a}_1 - 4 \vec{S}_1 \cdot \vec{v}_2 \vec{S}_2 \cdot \vec{v}_1 + 4 \vec{S}_1 \cdot \vec{S}_2 \vec{v}_1 \cdot \vec{v}_2 \Big) + \frac{1}{\rho^3} \\ & \left( 2 \vec{S}_1 \cdot \vec{S}_2 (\hat{n} \cdot \vec{v}_2)^3 - 2 \hat{n} \cdot \vec{S}_2 \vec{S}_1 \cdot \vec{v}_2 (\hat{n} \cdot \vec{v}_2)^2 - 6 \hat{n} \times \vec{S}_1 \cdot \vec{v}_1 \hat{n} \times \vec{S}_2 \cdot \vec{a}_1 \hat{n} \cdot \vec{v}_2 - 6 \hat{n} \times \vec{S}_1 \cdot \vec{v}_1 \hat{n} \times \vec{S}_2 \cdot \vec{v}_1 \hat{n} \cdot \vec{v}_2 - \right. \\ & 6 \hat{n} \times \vec{S}_1 \cdot \vec{a}_1 \hat{n} \times \vec{S}_2 \cdot \vec{v}_1 \hat{n} \cdot \vec{v}_2 - 6 \hat{n} \times \vec{S}_1 \cdot \vec{v}_2 \hat{n} \times \vec{S}_2 \cdot \vec{v}_2 \hat{n} \cdot \vec{v}_2 + 2 (\hat{n} \cdot \vec{v}_1)^2 \vec{S}_1 \cdot \vec{S}_2 \hat{n} \cdot \vec{v}_2 + 4 \hat{n} \cdot \vec{a}_1 \hat{n} \cdot \vec{v}_1 \vec{S}_1 \cdot \vec{S}_2 \hat{n} \cdot \vec{v}_2 + \\ & \frac{3}{2} \vec{S}_2 \cdot \vec{v}_1 \vec{S}_1 \cdot \vec{v}_2 \hat{n} \cdot \vec{v}_2 - 2 \hat{n} \cdot \vec{S}_1 \hat{n} \cdot \vec{v}_1 \vec{S}_2 \cdot \vec{a}_1 \hat{n} \cdot \vec{v}_2 - \vec{S}_1 \cdot \vec{v}_1 \vec{S}_2 \cdot \vec{a}_1 \hat{n} \cdot \vec{v}_2 - 2 \hat{n} \cdot \vec{a}_1 \hat{n} \cdot \vec{S}_1 \vec{S}_2 \cdot \vec{v}_1 \hat{n} \cdot \vec{v}_2 - \\ & 2 \hat{n} \cdot \vec{S}_1 \hat{n} \cdot \vec{v}_1 \vec{S}_2 \cdot \vec{v}_1 \hat{n} \cdot \vec{v}_2 - \vec{S}_1 \cdot \vec{v}_1 \vec{S}_2 \cdot \vec{v}_1 \hat{n} \cdot \vec{v}_2 - \vec{S}_1 \cdot \vec{a}_1 \vec{S}_2 \cdot \vec{v}_1 \hat{n} \cdot \vec{v}_2 + 2 \vec{S}_1 \cdot \vec{a}_2 \vec{S}_2 \cdot \vec{v}_1 \hat{n} \cdot \vec{v}_2 - \\ & \frac{1}{2} \vec{S}_1 \cdot \vec{v}_2 \vec{S}_2 \cdot \vec{v}_2 \hat{n} \cdot \vec{v}_2 - 36 \hat{n} \cdot \vec{S}_1 \hat{n} \cdot \vec{S}_2 \vec{v}_1 \cdot \vec{a}_1 \hat{n} \cdot \vec{v}_2 + 2 \vec{S}_1 \cdot \vec{S}_2 \vec{v}_1 \cdot \vec{a}_1 \hat{n} \cdot \vec{v}_2 - 2 \vec{S}_1 \cdot \vec{S}_2 \vec{v}_1 \cdot \vec{a}_2 \hat{n} \cdot \vec{v}_2 + \\ & 6 \hat{n} \cdot \vec{S}_1 \hat{n} \cdot \vec{S}_2 \vec{v}_1 \cdot \vec{v}_1 \hat{n} \cdot \vec{v}_2 + \vec{S}_1 \cdot \vec{S}_2 \vec{v}_1 \cdot \vec{v}_1 \hat{n} \cdot \vec{v}_2 - \frac{3}{2} \vec{S}_1 \cdot \vec{S}_2 \vec{v}_1 \cdot \vec{v}_2 \hat{n} \cdot \vec{v}_2 + \frac{7}{2} \hat{n} \times \vec{S}_2 \cdot \vec{v}_1 \vec{S}_1 \times \vec{v}_1 \cdot \vec{v}_2 + \\ & \frac{7}{2} \hat{n} \times \vec{S}_2 \cdot \vec{v}_1 \vec{S}_1 \times \vec{a}_1 \cdot \vec{v}_2 - \hat{n} \times \vec{S}_2 \cdot \vec{v}_2 \vec{S}_1 \times \vec{v}_1 \cdot \vec{a}_2 - \frac{3}{2} \hat{n} \times \vec{S}_2 \cdot \vec{v}_2 \vec{S}_1 \times \vec{v}_1 \cdot \vec{v}_2 + \frac{7}{2} \hat{n} \times \vec{S}_2 \cdot \vec{a}_1 \vec{S}_1 \times \vec{v}_1 \cdot \vec{v}_2 - \\ & 2 \hat{n} \times \vec{S}_2 \cdot \vec{a}_2 \vec{S}_1 \times \vec{v}_1 \cdot \vec{v}_2 + \frac{3}{2} \hat{n} \times \vec{S}_1 \cdot \vec{v}_1 \vec{S}_2 \times \vec{a}_1 \cdot \vec{v}_2 + \frac{3}{2} \hat{n} \times \vec{S}_1 \cdot \vec{v}_1 \vec{S}_2 \times \vec{v}_1 \cdot \vec{v}_2 + \frac{3}{2} \hat{n} \times \vec{S}_1 \cdot \vec{a}_1 \vec{S}_2 \times \vec{v}_1 \cdot \vec{v}_2 - \\ & 3 \hat{n} \cdot \vec{v}_1 \vec{a}_1 \cdot \vec{v}_2 \vec{S}_1 \cdot \vec{S}_2 + \frac{1}{2} \hat{n} \cdot \vec{v}_1 \vec{S}_1 \cdot \vec{v}_2 \vec{S}_2 \cdot \vec{a}_1 + \frac{1}{2} \hat{n} \cdot \vec{v}_1 \vec{S}_1 \cdot \vec{v}_2 \vec{S}_2 \cdot \vec{v}_1 + \frac{5}{2} \hat{n} \cdot \vec{S}_1 \vec{a}_1 \cdot \vec{v}_2 \vec{S}_2 \cdot \vec{v}_1 + \\ & \frac{1}{2} \hat{n} \cdot \vec{a}_1 \vec{S}_1 \cdot \vec{v}_2 \vec{S}_2 \cdot \vec{v}_1 + \hat{n} \cdot \vec{a}_2 \vec{S}_1 \cdot \vec{v}_2 \vec{S}_2 \cdot \vec{v}_1 + 9 \hat{n} \cdot \vec{S}_2 \vec{S}_1 \cdot \vec{v}_2 \vec{v}_1 \cdot \vec{a}_1 + 9 \hat{n} \cdot \vec{S}_1 \vec{S}_2 \cdot \vec{v}_2 \vec{v}_1 \cdot \vec{a}_1 - \\ & \frac{3}{2} \hat{n} \cdot \vec{S}_2 \vec{S}_1 \cdot \vec{v}_2 \vec{v}_1 \cdot \vec{v}_1 - \frac{3}{2} \hat{n} \cdot \vec{S}_1 \vec{S}_2 \cdot \vec{v}_2 \vec{v}_1 \cdot \vec{v}_1 - 3 \hat{n} \cdot \vec{v}_1 \vec{S}_1 \cdot \vec{S}_2 \vec{v}_1 \cdot \vec{v}_2 - 3 \hat{n} \cdot \vec{a}_1 \vec{S}_1 \cdot \vec{S}_2 \vec{v}_1 \cdot \vec{v}_2 - \\ & \hat{n} \cdot \vec{a}_2 \vec{S}_1 \cdot \vec{S}_2 \vec{v}_1 \cdot \vec{v}_2 + \frac{5}{2} \hat{n} \cdot \vec{S}_1 \vec{S}_2 \cdot \vec{a}_1 \vec{v}_1 \cdot \vec{v}_2 + \frac{5}{2} \hat{n} \cdot \vec{S}_1 \vec{S}_2 \cdot \vec{v}_1 \vec{v}_1 \cdot \vec{v}_2 + \frac{1}{2} \hat{n} \cdot \vec{S}_2 \vec{S}_1 \cdot \vec{v}_2 \vec{v}_2 \cdot \vec{v}_2 \Big) + \\ & \frac{1}{\rho^4} \left( 8 \vec{S}_1 \cdot \vec{S}_2 \vec{v}_1 \cdot \vec{v}_2 (\hat{n} \cdot \vec{v}_1)^2 - 8 \hat{n} \times \vec{S}_2 \cdot \vec{v}_1 \vec{S}_1 \times \vec{v}_1 \cdot \vec{v}_2 \hat{n} \cdot \vec{v}_1 + 4 \hat{n} \cdot \vec{v}_2 \vec{S}_1 \cdot \vec{S}_2 \vec{v}_1 \cdot \vec{v}_1 \hat{n} \cdot \vec{v}_1 - \right. \\ & 8 \hat{n} \cdot \vec{S}_1 \vec{S}_2 \cdot \vec{v}_1 \vec{v}_1 \cdot \vec{v}_2 \hat{n} \cdot \vec{v}_1 - 6 \hat{n} \times \vec{S}_2 \cdot \vec{v}_2 \vec{S}_1 \times \vec{v}_1 \cdot \vec{v}_2 \hat{n} \cdot \vec{v}_2 + 2 (\hat{n} \cdot \vec{v}_2)^2 \vec{S}_1 \cdot \vec{v}_2 \vec{S}_2 \cdot \vec{v}_1 - \\ & 4 \hat{n} \cdot \vec{S}_1 \hat{n} \cdot \vec{v}_2 \vec{S}_2 \cdot \vec{v}_1 \vec{v}_1 \cdot \vec{v}_1 + \vec{S}_1 \cdot \vec{v}_2 \vec{S}_2 \cdot \vec{v}_1 \vec{v}_1 \cdot \vec{v}_1 - 2 (\hat{n} \cdot \vec{v}_2)^2 \vec{S}_1 \cdot \vec{S}_2 \vec{v}_1 \cdot \vec{v}_2 + 2 \vec{S}_1 \cdot \vec{v}_1 \vec{S}_2 \cdot \vec{v}_1 \vec{v}_1 \cdot \vec{v}_2 - \\ & \left. 3 \vec{S}_1 \cdot \vec{S}_2 \vec{v}_1 \cdot \vec{v}_1 \vec{v}_1 \cdot \vec{v}_2 - \frac{1}{2} \vec{S}_1 \cdot \vec{v}_2 \vec{S}_2 \cdot \vec{v}_1 \vec{v}_2 \cdot \vec{v}_2 + \frac{1}{2} \vec{S}_1 \cdot \vec{S}_2 \vec{v}_1 \cdot \vec{v}_2 \vec{v}_2 \cdot \vec{v}_2 \right) \Big) m_1 \Big\} \end{aligned}$$

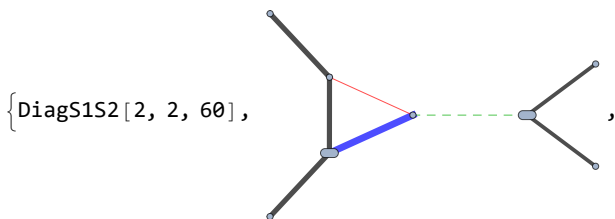

$$\begin{aligned} G^2 \left( \frac{1}{r^2} \right. & \left( -6 \frac{1}{S_1} \cdot \frac{1}{S_2} (\hat{n} \cdot \vec{v}_1)^2 + 8 \hat{n} \cdot \vec{S}_1 \frac{1}{S_2} \cdot \vec{a}_1 \hat{n} \cdot \vec{v}_1 + 6 \hat{n} \cdot \vec{S}_1 \frac{1}{S_2} \cdot \vec{v}_1 \hat{n} \cdot \vec{v}_1 - 2 \hat{n} \cdot \vec{S}_2 \vec{S}_1 \cdot \frac{1}{a_2} \hat{n} \cdot \vec{v}_1 - 12 \hat{n} \cdot \vec{a}_1 \vec{S}_1 \cdot \frac{1}{S_2} \hat{n} \cdot \vec{v}_1 + \right. \\ & 4 \hat{n} \cdot \vec{a}_2 \vec{S}_1 \cdot \frac{1}{S_2} \hat{n} \cdot \vec{v}_1 + 2 \hat{n} \cdot \vec{v}_2 \vec{S}_1 \cdot \frac{1}{S_2} \hat{n} \cdot \vec{v}_1 - 4 \hat{n} \cdot \vec{S}_2 \vec{S}_1 \cdot \vec{a}_2 \hat{n} \cdot \vec{v}_1 + 2 \hat{n} \cdot \vec{a}_2 \vec{S}_1 \cdot \vec{S}_2 \hat{n} \cdot \vec{v}_1 - 2 \hat{n} \cdot \vec{S}_2 \vec{S}_1 \cdot \vec{v}_2 \hat{n} \cdot \vec{v}_1 + \\ & 6 \hat{n} \times \vec{S}_1 \cdot \vec{v}_1 \hat{n} \times \vec{S}_2 \cdot \vec{v}_1 + 8 \hat{n} \times \vec{S}_2 \cdot \vec{v}_1 \hat{n} \times \vec{S}_1 \cdot \vec{a}_1 + 4 \hat{n} \times \vec{S}_2 \cdot \vec{a}_1 \hat{n} \times \vec{S}_1 \cdot \vec{v}_1 + 4 \hat{n} \cdot \vec{a}_1 \hat{n} \cdot \vec{S}_1 \frac{1}{S_2} \cdot \vec{v}_1 + \\ & \left. 4 \frac{1}{S_2} \cdot \vec{v}_1 \vec{S}_1 \cdot \vec{a}_2 + 2 \frac{1}{S_2} \cdot \vec{v}_1 \vec{S}_1 \cdot \vec{v}_2 + 2 \vec{S}_1 \cdot \frac{1}{a_2} \vec{S}_2 \cdot \vec{v}_1 - 2 \vec{S}_1 \cdot \vec{S}_2 \vec{v}_1 \cdot \frac{1}{a_2} - 4 \vec{S}_1 \cdot \frac{1}{S_2} \vec{v}_1 \cdot \vec{a}_2 - 2 \vec{S}_1 \cdot \vec{S}_2 \vec{v}_1 \cdot \vec{v}_2 \right) + \\ & \left. \frac{1}{r^3} \left( 24 \frac{1}{S_1} \cdot \vec{S}_2 (\hat{n} \cdot \vec{v}_1)^3 + 2 \vec{S}_1 \cdot \frac{1}{S_2} (\hat{n} \cdot \vec{v}_1)^3 - 24 \hat{n} \cdot \vec{v}_2 \vec{S}_1 \cdot \vec{S}_2 (\hat{n} \cdot \vec{v}_1)^2 - 2 \hat{n} \cdot \vec{S}_1 \frac{1}{S_2} \cdot \vec{v}_1 (\hat{n} \cdot \vec{v}_1)^2 - \right. \right. \end{aligned}$$



$$\begin{aligned}
& 2 \hat{n} \cdot \vec{S}_2 \hat{n} \cdot \vec{v}_2 \vec{S}_1 \cdot \vec{v}_2 \vec{v}_1 \cdot \vec{v}_1 - 8 \hat{n} \cdot \vec{S}_1 \hat{n} \cdot \vec{v}_2 \vec{S}_2 \cdot \vec{v}_1 \vec{v}_1 \cdot \vec{v}_1 - 3 \vec{S}_1 \cdot \vec{v}_1 \vec{S}_2 \cdot \vec{v}_1 \vec{v}_1 \cdot \vec{v}_1 + 2 \vec{S}_1 \cdot \vec{v}_2 \vec{S}_2 \cdot \vec{v}_1 \vec{v}_1 \cdot \vec{v}_1 + \\
& \frac{3}{2} \vec{S}_1 \cdot \vec{v}_1 \vec{S}_2 \cdot \vec{v}_2 \vec{v}_1 \cdot \vec{v}_1 - \vec{S}_1 \cdot \vec{v}_2 \vec{S}_2 \cdot \vec{v}_2 \vec{v}_1 \cdot \vec{v}_1 + 6 \hat{n} \times \vec{S}_1 \cdot \vec{v}_1 \hat{n} \times \vec{S}_2 \cdot \vec{v}_1 \vec{v}_1 \cdot \vec{v}_2 + 6 \hat{n} \times \vec{S}_1 \cdot \vec{v}_1 \hat{n} \times \vec{S}_2 \cdot \vec{v}_2 \vec{v}_1 \cdot \vec{v}_2 + \\
& 6 \hat{n} \times \vec{S}_1 \cdot \vec{v}_2 \hat{n} \times \vec{S}_2 \cdot \vec{v}_2 \vec{v}_1 \cdot \vec{v}_2 - 8 (\hat{n} \cdot \vec{v}_2)^2 \vec{S}_1 \cdot \vec{S}_2 \vec{v}_1 \cdot \vec{v}_2 + 4 \hat{n} \cdot \vec{S}_2 \hat{n} \cdot \vec{v}_2 \vec{S}_1 \cdot \vec{v}_2 \vec{v}_1 \cdot \vec{v}_2 + \\
& \frac{1}{2} \vec{S}_1 \cdot \vec{v}_1 \vec{S}_2 \cdot \vec{v}_1 \vec{v}_1 \cdot \vec{v}_2 + 3 \vec{S}_1 \cdot \vec{v}_2 \vec{S}_2 \cdot \vec{v}_1 \vec{v}_1 \cdot \vec{v}_2 + \frac{1}{2} \vec{S}_1 \cdot \vec{v}_2 \vec{S}_2 \cdot \vec{v}_2 \vec{v}_1 \cdot \vec{v}_2 - 6 \hat{n} \cdot \vec{S}_1 \hat{n} \cdot \vec{S}_2 \vec{v}_1 \cdot \vec{v}_1 \vec{v}_1 \cdot \vec{v}_2 - \\
& \vec{S}_1 \cdot \vec{S}_2 \vec{v}_1 \cdot \vec{v}_1 \vec{v}_1 \cdot \vec{v}_2 - \vec{S}_1 \cdot \vec{v}_2 \vec{S}_2 \cdot \vec{v}_1 \vec{v}_2 \cdot \vec{v}_2 + \vec{S}_1 \cdot \vec{S}_2 \vec{v}_1 \cdot \vec{v}_1 \vec{v}_2 \cdot \vec{v}_2 + \frac{1}{2} \vec{S}_1 \cdot \vec{S}_2 \vec{v}_1 \cdot \vec{v}_2 \vec{v}_2 \cdot \vec{v}_2 \Big) \Big) m_1 \Big\}
\end{aligned}$$

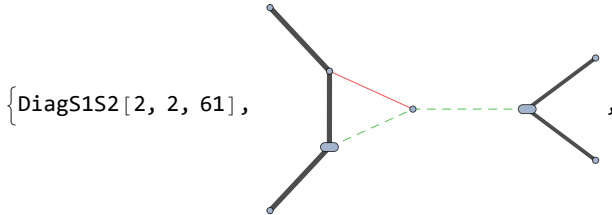

$$\begin{aligned}
& G^2 \left( \frac{1}{r^2} \left( 8 \vec{S}_1 \cdot \vec{v}_2 \vec{S}_2 \cdot \vec{v}_1 - 8 \vec{a}_1 \cdot \vec{v}_2 \vec{S}_1 \cdot \vec{S}_2 - 8 \vec{a}_1 \cdot \vec{a}_2 \vec{S}_1 \cdot \vec{S}_2 + 8 \vec{S}_2 \cdot \vec{a}_1 \vec{S}_1 \cdot \vec{v}_2 + \right. \right. \\
& \left. \left. 8 \vec{S}_1 \cdot \vec{a}_2 \vec{S}_2 \cdot \vec{a}_1 + 8 \vec{S}_1 \cdot \vec{a}_2 \vec{S}_2 \cdot \vec{v}_1 - 8 \vec{S}_1 \cdot \vec{S}_2 \vec{v}_1 \cdot \vec{a}_2 - 8 \vec{S}_1 \cdot \vec{S}_2 \vec{v}_1 \cdot \vec{v}_2 \right) + \frac{1}{r^3} \right. \\
& \left( -12 \hat{n} \times \vec{S}_2 \cdot \vec{v}_2 \vec{S}_1 \times \vec{v}_1 \cdot \vec{v}_2 - 7 \hat{n} \times \vec{S}_1 \cdot \vec{v}_1 \vec{S}_2 \times \vec{v}_1 \cdot \vec{v}_2 - 12 \hat{n} \times \vec{S}_2 \cdot \vec{v}_2 \vec{S}_1 \times \vec{a}_1 \cdot \vec{v}_2 + 8 \hat{n} \times \vec{S}_2 \cdot \vec{v}_1 \vec{S}_1 \times \vec{v}_1 \cdot \vec{a}_1 - \right. \\
& 7 \hat{n} \times \vec{S}_1 \cdot \vec{v}_1 \vec{S}_2 \times \vec{v}_1 \cdot \vec{a}_2 - 2 \hat{n} \times \vec{S}_1 \cdot \vec{v}_2 \vec{S}_2 \times \vec{v}_2 \cdot \vec{a}_2 - 4 \hat{n} \cdot \vec{v}_2 \vec{a}_1 \cdot \vec{v}_2 \vec{S}_1 \cdot \vec{S}_2 - 5 \hat{n} \cdot \vec{v}_1 \vec{S}_2 \cdot \vec{v}_1 \vec{S}_1 \cdot \vec{v}_2 + \\
& 4 \hat{n} \cdot \vec{v}_2 \vec{S}_1 \cdot \vec{v}_2 \vec{S}_2 \cdot \vec{a}_1 + 4 \hat{n} \cdot \vec{v}_2 \vec{S}_1 \cdot \vec{v}_2 \vec{S}_2 \cdot \vec{v}_1 - 5 \hat{n} \cdot \vec{v}_1 \vec{S}_1 \cdot \vec{a}_2 \vec{S}_2 \cdot \vec{v}_1 + 8 \hat{n} \cdot \vec{v}_1 \vec{S}_1 \cdot \vec{S}_2 \vec{v}_1 \cdot \vec{a}_1 - 8 \hat{n} \cdot \vec{S}_1 \vec{S}_2 \cdot \vec{v}_1 \\
& \vec{v}_1 \cdot \vec{a}_1 + 5 \hat{n} \cdot \vec{v}_1 \vec{S}_1 \cdot \vec{S}_2 \vec{v}_1 \cdot \vec{a}_2 + 16 \hat{n} \cdot \vec{v}_1 \vec{S}_1 \cdot \vec{S}_2 \vec{v}_1 \cdot \vec{v}_1 - 3 \hat{n} \cdot \vec{v}_2 \vec{S}_1 \cdot \vec{S}_2 \vec{v}_1 \cdot \vec{v}_1 + 3 \hat{n} \cdot \vec{S}_2 \vec{S}_1 \cdot \vec{a}_2 \vec{v}_1 \cdot \vec{v}_1 + \\
& 16 \hat{n} \cdot \vec{a}_1 \vec{S}_1 \cdot \vec{S}_2 \vec{v}_1 \cdot \vec{v}_1 - 3 \hat{n} \cdot \vec{a}_2 \vec{S}_1 \cdot \vec{S}_2 \vec{v}_1 \cdot \vec{v}_1 + 3 \hat{n} \cdot \vec{S}_2 \vec{S}_1 \cdot \vec{v}_2 \vec{v}_1 \cdot \vec{v}_1 - 16 \hat{n} \cdot \vec{S}_1 \vec{S}_2 \cdot \vec{a}_1 \vec{v}_1 \cdot \vec{v}_1 - \\
& 16 \hat{n} \cdot \vec{S}_1 \vec{S}_2 \cdot \vec{v}_1 \vec{v}_1 \cdot \vec{v}_1 - 4 \hat{n} \cdot \vec{v}_2 \vec{S}_1 \cdot \vec{S}_2 \vec{v}_1 \cdot \vec{v}_2 + 5 \hat{n} \cdot \vec{v}_1 \vec{S}_1 \cdot \vec{S}_2 \vec{v}_1 \cdot \vec{v}_2 - 2 \hat{n} \cdot \vec{v}_2 \vec{S}_1 \cdot \vec{S}_2 \vec{v}_2 \cdot \vec{a}_2 + \\
& 2 \hat{n} \cdot \vec{S}_2 \vec{S}_1 \cdot \vec{v}_2 \vec{v}_2 \cdot \vec{a}_2 - \hat{n} \cdot \vec{v}_2 \vec{S}_1 \cdot \vec{S}_2 \vec{v}_2 \cdot \vec{v}_2 + \hat{n} \cdot \vec{S}_2 \vec{S}_1 \cdot \vec{a}_2 \vec{v}_2 \cdot \vec{v}_2 - \hat{n} \cdot \vec{a}_2 \vec{S}_1 \cdot \vec{S}_2 \vec{v}_2 \cdot \vec{v}_2 + \hat{n} \cdot \vec{S}_2 \vec{S}_1 \cdot \vec{v}_2 \vec{v}_2 \cdot \vec{v}_2 \Big) + \\
& \frac{1}{r^4} \left( -\frac{39}{2} \vec{S}_1 \cdot \vec{S}_2 \vec{v}_1 \cdot \vec{v}_1 (\hat{n} \cdot \vec{v}_1)^2 + 15 \hat{n} \times \vec{S}_2 \cdot \vec{v}_2 \vec{S}_1 \times \vec{v}_1 \cdot \vec{v}_2 \hat{n} \cdot \vec{v}_1 - 5 \hat{n} \cdot \vec{v}_2 \vec{S}_1 \cdot \vec{v}_2 \vec{S}_2 \cdot \vec{v}_1 \hat{n} \cdot \vec{v}_1 + \right. \\
& \frac{39}{2} \hat{n} \cdot \vec{S}_1 \vec{S}_2 \cdot \vec{v}_1 \vec{v}_1 \cdot \vec{v}_1 \hat{n} \cdot \vec{v}_1 + 5 \hat{n} \cdot \vec{v}_2 \vec{S}_1 \cdot \vec{S}_2 \vec{v}_1 \cdot \vec{v}_2 \hat{n} \cdot \vec{v}_1 - \frac{7}{2} \hat{n} \cdot \vec{S}_1 \hat{n} \cdot \vec{S}_2 (\vec{v}_1 \cdot \vec{v}_1)^2 - \\
& \frac{1}{2} \vec{S}_1 \cdot \vec{S}_2 (\vec{v}_1 \cdot \vec{v}_1)^2 - \frac{13}{2} \vec{S}_1 \cdot \vec{S}_2 (\vec{v}_1 \cdot \vec{v}_2)^2 - \frac{3}{4} \vec{S}_1 \cdot \vec{S}_2 (\vec{v}_2 \cdot \vec{v}_2)^2 + \frac{11}{2} \vec{S}_1 \times \vec{v}_1 \cdot \vec{v}_2 \vec{S}_2 \times \vec{v}_1 \cdot \vec{v}_2 - \\
& 7 \hat{n} \times \vec{S}_1 \cdot \vec{v}_1 \vec{S}_2 \times \vec{v}_1 \cdot \vec{v}_2 \hat{n} \cdot \vec{v}_2 + \frac{57}{2} \hat{n} \times \vec{S}_1 \cdot \vec{v}_1 \hat{n} \times \vec{S}_2 \cdot \vec{v}_1 \vec{v}_1 \cdot \vec{v}_1 + 9 \hat{n} \times \vec{S}_1 \cdot \vec{v}_2 \hat{n} \times \vec{S}_2 \cdot \vec{v}_2 \vec{v}_1 \cdot \vec{v}_1 - \\
& 3 (\hat{n} \cdot \vec{v}_2)^2 \vec{S}_1 \cdot \vec{S}_2 \vec{v}_1 \cdot \vec{v}_1 + 3 \hat{n} \cdot \vec{S}_2 \hat{n} \cdot \vec{v}_2 \vec{S}_1 \cdot \vec{v}_2 \vec{v}_1 \cdot \vec{v}_1 + \frac{9}{4} \vec{S}_1 \cdot \vec{v}_1 \vec{S}_2 \cdot \vec{v}_1 \vec{v}_1 \cdot \vec{v}_1 + \frac{3}{2} \vec{S}_1 \cdot \vec{v}_2 \vec{S}_2 \cdot \vec{v}_2 \vec{v}_1 \cdot \vec{v}_1 + \\
& 21 \hat{n} \times \vec{S}_1 \cdot \vec{v}_1 \hat{n} \times \vec{S}_2 \cdot \vec{v}_2 \vec{v}_1 \cdot \vec{v}_2 + \frac{13}{2} \vec{S}_1 \cdot \vec{v}_2 \vec{S}_2 \cdot \vec{v}_1 \vec{v}_1 \cdot \vec{v}_2 + \frac{7}{2} \hat{n} \times \vec{S}_1 \cdot \vec{v}_2 \hat{n} \times \vec{S}_2 \cdot \vec{v}_2 \vec{v}_2 \cdot \vec{v}_2 - \\
& \left. \frac{1}{2} (\hat{n} \cdot \vec{v}_2)^2 \vec{S}_1 \cdot \vec{S}_2 \vec{v}_2 \cdot \vec{v}_2 + \frac{1}{2} \hat{n} \cdot \vec{S}_2 \hat{n} \cdot \vec{v}_2 \vec{S}_1 \cdot \vec{v}_2 \vec{v}_2 \cdot \vec{v}_2 + \frac{3}{4} \vec{S}_1 \cdot \vec{v}_2 \vec{S}_2 \cdot \vec{v}_2 \vec{v}_2 \cdot \vec{v}_2 - \frac{3}{2} \vec{S}_1 \cdot \vec{S}_2 \vec{v}_1 \cdot \vec{v}_1 \vec{v}_2 \cdot \vec{v}_2 \right) \Big) m_1 \Big\}
\end{aligned}$$

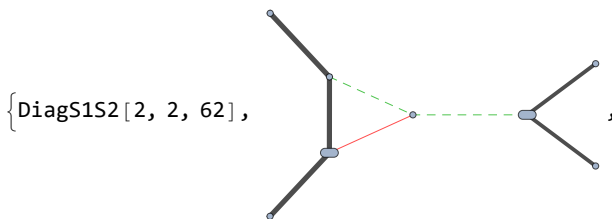





$$\begin{aligned}
& 4 \hat{n} \cdot \vec{S}_1 \vec{S}_2 \cdot \vec{v}_1 \vec{v}_1 \cdot \vec{v}_2 \hat{n} \cdot \vec{v}_1 + 2 \hat{n} \cdot \vec{S}_2 \vec{S}_1 \cdot \vec{v}_2 \vec{v}_2 \cdot \vec{v}_2 \hat{n} \cdot \vec{v}_1 + 72 \hat{n} \times \vec{S}_1 \cdot \vec{v}_1 \hat{n} \times \vec{S}_2 \cdot \vec{v}_2 (\hat{n} \cdot \vec{v}_2)^2 + \\
& \frac{9}{2} \vec{S}_1 \cdot \vec{S}_2 (\vec{v}_1 \cdot \vec{v}_1)^2 - \frac{7}{4} \vec{S}_1 \cdot \vec{S}_2 (\vec{v}_1 \cdot \vec{v}_2)^2 + \frac{13}{4} \vec{S}_1 \times \vec{v}_1 \cdot \vec{v}_2 \vec{S}_2 \times \vec{v}_1 \cdot \vec{v}_2 - 21 \hat{n} \times \vec{S}_2 \cdot \vec{v}_2 \vec{S}_1 \times \vec{v}_1 \cdot \vec{v}_2 \hat{n} \cdot \vec{v}_2 - \\
& 7 \hat{n} \times \vec{S}_1 \cdot \vec{v}_1 \vec{S}_2 \times \vec{v}_1 \cdot \vec{v}_2 \hat{n} \cdot \vec{v}_2 - 6 \hat{n} \times \vec{S}_1 \cdot \vec{v}_2 \vec{S}_2 \times \vec{v}_1 \cdot \vec{v}_2 \hat{n} \cdot \vec{v}_2 + 11 (\hat{n} \cdot \vec{v}_2)^2 \vec{S}_1 \cdot \vec{v}_2 \vec{S}_2 \cdot \vec{v}_1 - \\
& 6 \hat{n} \times \vec{S}_1 \cdot \vec{v}_1 \hat{n} \times \vec{S}_2 \cdot \vec{v}_1 \vec{v}_1 \cdot \vec{v}_1 - 6 \hat{n} \cdot \vec{S}_2 \hat{n} \cdot \vec{v}_2 \vec{S}_1 \cdot \vec{v}_1 \vec{v}_1 \cdot \vec{v}_1 - 2 \hat{n} \cdot \vec{S}_1 \hat{n} \cdot \vec{v}_2 \vec{S}_2 \cdot \vec{v}_1 \vec{v}_1 \cdot \vec{v}_1 - \frac{9}{2} \vec{S}_1 \cdot \vec{v}_1 \vec{S}_2 \cdot \vec{v}_1 \vec{v}_1 \cdot \vec{v}_1 + \\
& \frac{1}{2} \vec{S}_1 \cdot \vec{v}_2 \vec{S}_2 \cdot \vec{v}_1 \vec{v}_1 \cdot \vec{v}_1 + \frac{3}{2} \vec{S}_1 \cdot \vec{v}_1 \vec{S}_2 \cdot \vec{v}_2 \vec{v}_1 \cdot \vec{v}_1 + 14 \hat{n} \times \vec{S}_1 \cdot \vec{v}_1 \hat{n} \times \vec{S}_2 \cdot \vec{v}_1 \vec{v}_1 \cdot \vec{v}_2 + 5 \hat{n} \times \vec{S}_1 \cdot \vec{v}_1 \hat{n} \times \vec{S}_2 \cdot \vec{v}_2 \vec{v}_1 \cdot \vec{v}_2 + \\
& 6 \hat{n} \times \vec{S}_1 \cdot \vec{v}_2 \hat{n} \times \vec{S}_2 \cdot \vec{v}_2 \vec{v}_1 \cdot \vec{v}_2 - 15 (\hat{n} \cdot \vec{v}_2)^2 \vec{S}_1 \cdot \vec{S}_2 \vec{v}_1 \cdot \vec{v}_2 + 4 \hat{n} \cdot \vec{S}_2 \hat{n} \cdot \vec{v}_2 \vec{S}_1 \cdot \vec{v}_2 \vec{v}_1 \cdot \vec{v}_2 + \\
& \frac{9}{2} \vec{S}_1 \cdot \vec{v}_1 \vec{S}_2 \cdot \vec{v}_1 \vec{v}_1 \cdot \vec{v}_2 + \frac{7}{4} \vec{S}_1 \cdot \vec{v}_2 \vec{S}_2 \cdot \vec{v}_1 \vec{v}_1 \cdot \vec{v}_2 + \frac{1}{2} \vec{S}_1 \cdot \vec{v}_2 \vec{S}_2 \cdot \vec{v}_2 \vec{v}_1 \cdot \vec{v}_2 - 6 \hat{n} \cdot \vec{S}_1 \hat{n} \cdot \vec{S}_2 \vec{v}_1 \cdot \vec{v}_1 \vec{v}_1 \cdot \vec{v}_2 - \\
& \frac{7}{2} \vec{S}_1 \cdot \vec{S}_2 \vec{v}_1 \cdot \vec{v}_1 \vec{v}_1 \cdot \vec{v}_2 - 12 \hat{n} \times \vec{S}_1 \cdot \vec{v}_1 \hat{n} \times \vec{S}_2 \cdot \vec{v}_2 \vec{v}_2 \cdot \vec{v}_2 - \frac{11}{4} \vec{S}_1 \cdot \vec{v}_2 \vec{S}_2 \cdot \vec{v}_1 \vec{v}_2 \cdot \vec{v}_2 + \frac{9}{4} \vec{S}_1 \cdot \vec{S}_2 \vec{v}_1 \cdot \vec{v}_2 \vec{v}_2 \cdot \vec{v}_2 \Big) \Big) m_1 \Big\}
\end{aligned}$$

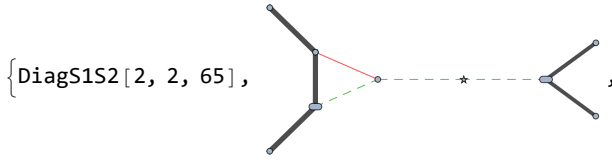

$$\begin{aligned}
& G^2 \left( \frac{1}{r} \left( \hat{n} \cdot \vec{S}_2 \vec{S}_1 \cdot \frac{1}{a_2} + 8 \hat{n} \cdot \vec{a}_1 \vec{S}_1 \cdot \frac{1}{S_2} - 2 \hat{n} \cdot \vec{a}_2 \vec{S}_1 \cdot \frac{1}{S_2} - \hat{n} \cdot \vec{v}_2 \vec{S}_1 \cdot \frac{1}{S_2} + 2 \hat{n} \cdot \vec{S}_2 \vec{S}_1 \cdot \vec{a}_2 - \hat{n} \cdot \vec{a}_2 \vec{S}_1 \cdot \vec{S}_2 + \right. \right. \\
& \quad \left. \hat{n} \cdot \vec{S}_2 \vec{S}_1 \cdot \vec{v}_2 + 4 \hat{n} \cdot \vec{v}_1 \vec{S}_1 \cdot \frac{1}{S_2} - 4 \hat{n} \cdot \vec{S}_1 \vec{S}_2 \cdot \vec{a}_1 - 8 \hat{n} \cdot \vec{S}_1 \vec{S}_2 \cdot \vec{a}_1 - 4 \hat{n} \cdot \vec{S}_1 \vec{S}_2 \cdot \vec{v}_1 + 4 \hat{n} \cdot \vec{a}_1 \vec{S}_1 \cdot \frac{1}{S_2} \right) + \frac{1}{r^2} \\
& \quad \left( -\frac{21}{2} \vec{S}_1 \cdot \vec{S}_2 (\hat{n} \cdot \vec{v}_1)^2 + 8 \hat{n} \cdot \vec{v}_2 \vec{S}_1 \cdot \vec{S}_2 \hat{n} \cdot \vec{v}_1 + \frac{21}{2} \hat{n} \cdot \vec{S}_1 \vec{S}_2 \cdot \vec{a}_1 \hat{n} \cdot \vec{v}_1 + \frac{21}{2} \hat{n} \cdot \vec{S}_1 \vec{S}_2 \cdot \vec{v}_1 \hat{n} \cdot \vec{v}_1 - 2 \hat{n} \cdot \vec{S}_2 \vec{S}_1 \cdot \frac{1}{a_2} \hat{n} \cdot \vec{v}_1 - \right. \\
& \quad 13 \hat{n} \cdot \vec{a}_1 \vec{S}_1 \cdot \frac{1}{S_2} \hat{n} \cdot \vec{v}_1 + 4 \hat{n} \cdot \vec{a}_2 \vec{S}_1 \cdot \frac{1}{S_2} \hat{n} \cdot \vec{v}_1 + 2 \hat{n} \cdot \vec{v}_2 \vec{S}_1 \cdot \frac{1}{S_2} \hat{n} \cdot \vec{v}_1 - 4 \hat{n} \cdot \vec{S}_2 \vec{S}_1 \cdot \vec{a}_2 \hat{n} \cdot \vec{v}_1 + 2 \hat{n} \cdot \vec{a}_2 \vec{S}_1 \cdot \vec{S}_2 \hat{n} \cdot \vec{v}_1 - \\
& \quad 2 \hat{n} \cdot \vec{S}_2 \vec{S}_1 \cdot \vec{v}_2 \hat{n} \cdot \vec{v}_1 + \frac{7}{2} \hat{n} \times \vec{S}_1 \cdot \vec{v}_1 \hat{n} \times \vec{S}_2 \cdot \vec{v}_1 + \frac{3}{2} \hat{n} \times \vec{S}_1 \cdot \vec{v}_2 \hat{n} \times \vec{S}_2 \cdot \vec{v}_2 + \frac{7}{2} \hat{n} \times \vec{S}_2 \cdot \vec{v}_1 \hat{n} \times \vec{S}_1 \cdot \vec{a}_1 + \\
& \quad \frac{7}{2} \hat{n} \times \vec{S}_2 \cdot \vec{a}_1 \hat{n} \times \vec{S}_1 \cdot \vec{v}_1 + \frac{3}{2} \hat{n} \times \vec{S}_1 \cdot \vec{v}_2 \hat{n} \times \vec{S}_2 \cdot \vec{a}_2 + \frac{3}{2} \hat{n} \times \vec{S}_1 \cdot \vec{a}_2 \hat{n} \times \vec{S}_2 \cdot \vec{v}_2 - \frac{5}{2} (\hat{n} \cdot \vec{v}_2)^2 \vec{S}_1 \cdot \frac{1}{S_2} + \\
& \quad \frac{5}{2} \hat{n} \cdot \vec{S}_2 \hat{n} \cdot \vec{v}_2 \vec{S}_1 \cdot \vec{a}_2 + 16 \hat{n} \cdot \vec{a}_1 \hat{n} \cdot \vec{v}_2 \vec{S}_1 \cdot \vec{S}_2 - 3 \hat{n} \cdot \vec{a}_2 \hat{n} \cdot \vec{v}_2 \vec{S}_1 \cdot \vec{S}_2 + \frac{1}{2} \hat{n} \cdot \vec{a}_2 \hat{n} \cdot \vec{S}_2 \vec{S}_1 \cdot \vec{v}_2 + \frac{5}{2} \hat{n} \cdot \vec{S}_2 \hat{n} \cdot \vec{v}_2 \vec{S}_1 \cdot \vec{v}_2 + \\
& \quad \frac{5}{2} \hat{n} \cdot \vec{a}_1 \hat{n} \cdot \vec{S}_1 \vec{S}_2 \cdot \vec{v}_1 - \frac{7}{2} \vec{S}_1 \cdot \vec{v}_1 \vec{S}_2 \cdot \vec{v}_1 - \frac{1}{2} \vec{S}_1 \cdot \vec{v}_2 \vec{S}_2 \cdot \vec{v}_2 - 8 \vec{S}_1 \cdot \vec{S}_2 \vec{a}_1 \cdot \vec{v}_2 + \frac{1}{2} \vec{S}_2 \cdot \vec{v}_1 \vec{S}_1 \cdot \vec{a}_1 + 2 \vec{S}_2 \cdot \vec{v}_1 \vec{S}_1 \cdot \vec{a}_2 + \\
& \quad 8 \hat{n} \cdot \vec{a}_1 \hat{n} \cdot \vec{v}_2 \vec{S}_1 \cdot \vec{S}_2 - 4 \vec{a}_1 \cdot \vec{v}_2 \vec{S}_1 \cdot \vec{S}_2 - \frac{7}{2} \vec{S}_2 \cdot \vec{a}_1 \vec{S}_1 \cdot \vec{v}_1 + \frac{2}{2} \vec{S}_2 \cdot \vec{v}_1 \vec{S}_1 \cdot \vec{v}_2 - 8 \hat{n} \cdot \vec{S}_1 \hat{n} \cdot \vec{v}_2 \vec{S}_2 \cdot \frac{1}{a_1} + 4 \vec{S}_1 \cdot \vec{v}_2 \vec{S}_2 \cdot \frac{1}{a_1} - \\
& \quad 16 \hat{n} \cdot \vec{S}_1 \hat{n} \cdot \vec{v}_2 \vec{S}_2 \cdot \vec{a}_1 + 8 \vec{S}_1 \cdot \vec{v}_2 \vec{S}_2 \cdot \vec{a}_1 + \frac{1}{2} \vec{S}_1 \cdot \vec{v}_2 \vec{S}_2 \cdot \vec{a}_2 - 8 \hat{n} \cdot \vec{S}_1 \hat{n} \cdot \vec{v}_2 \vec{S}_2 \cdot \vec{v}_1 + 4 \vec{S}_1 \cdot \vec{v}_2 \vec{S}_2 \cdot \vec{v}_1 + \\
& \quad \vec{S}_1 \cdot \frac{1}{a_2} \vec{S}_2 \cdot \vec{v}_1 - \frac{1}{2} \vec{S}_1 \cdot \vec{a}_2 \vec{S}_2 \cdot \vec{v}_2 - \vec{S}_1 \cdot \vec{S}_2 \vec{v}_1 \cdot \frac{1}{a_2} - 3 \hat{n} \cdot \vec{S}_2 \hat{n} \cdot \vec{S}_1 \vec{v}_1 \cdot \vec{a}_1 + 3 \vec{S}_1 \cdot \vec{S}_2 \vec{v}_1 \cdot \vec{a}_1 - 2 \vec{S}_1 \cdot \vec{S}_2 \vec{v}_1 \cdot \vec{a}_2 - \\
& \quad \frac{3}{2} \hat{n} \cdot \vec{S}_1 \hat{n} \cdot \frac{1}{S_2} \vec{v}_1 \cdot \vec{v}_1 + \frac{7}{2} \vec{S}_1 \cdot \frac{1}{S_2} \vec{v}_1 \cdot \vec{v}_1 - 4 \vec{S}_1 \cdot \vec{S}_2 \vec{v}_1 \cdot \vec{v}_2 - \vec{S}_1 \cdot \frac{2}{S_2} \vec{v}_1 \cdot \vec{v}_2 + \frac{1}{2} \vec{S}_1 \cdot \frac{1}{S_2} \vec{v}_2 \cdot \vec{v}_2 \Big) + \frac{1}{r^3} \\
& \quad \left( 10 \vec{S}_1 \cdot \vec{S}_2 (\hat{n} \cdot \vec{v}_1)^3 - 42 \hat{n} \cdot \vec{v}_2 \vec{S}_1 \cdot \vec{S}_2 (\hat{n} \cdot \vec{v}_1)^2 - 10 \hat{n} \cdot \vec{S}_1 \vec{S}_2 \cdot \vec{v}_1 (\hat{n} \cdot \vec{v}_1)^2 - 14 \hat{n} \times \vec{S}_2 \cdot \vec{v}_1 \hat{n} \times \vec{S}_1 \cdot \vec{v}_1 \hat{n} \cdot \vec{v}_1 - \right. \\
& \quad 6 \hat{n} \times \vec{S}_2 \cdot \vec{v}_2 \hat{n} \times \vec{S}_1 \cdot \vec{v}_2 \hat{n} \cdot \vec{v}_1 - 6 \hat{n} \times \vec{S}_1 \cdot \vec{v}_2 \hat{n} \times \vec{S}_2 \cdot \vec{a}_2 \hat{n} \cdot \vec{v}_1 - 6 \hat{n} \times \vec{S}_1 \cdot \vec{a}_2 \hat{n} \times \vec{S}_2 \cdot \vec{v}_2 \hat{n} \cdot \vec{v}_1 + \\
& \quad 10 (\hat{n} \cdot \vec{v}_2)^2 \vec{S}_1 \cdot \frac{1}{S_2} \hat{n} \cdot \vec{v}_1 - 10 \hat{n} \cdot \vec{S}_2 \hat{n} \cdot \vec{v}_2 \vec{S}_1 \cdot \vec{a}_2 \hat{n} \cdot \vec{v}_1 - 52 \hat{n} \cdot \vec{a}_1 \hat{n} \cdot \vec{v}_2 \vec{S}_1 \cdot \vec{S}_2 \hat{n} \cdot \vec{v}_1 + 12 \hat{n} \cdot \vec{a}_2 \hat{n} \cdot \vec{v}_2 \vec{S}_1 \cdot \vec{S}_2 \hat{n} \cdot \vec{v}_1 + \\
& \quad 13 \vec{a}_1 \cdot \vec{v}_2 \vec{S}_1 \cdot \vec{S}_2 \hat{n} \cdot \vec{v}_1 + \frac{3}{2} \vec{S}_2 \cdot \vec{v}_1 \vec{S}_1 \cdot \vec{v}_1 \hat{n} \cdot \vec{v}_1 - 2 \hat{n} \cdot \vec{a}_2 \hat{n} \cdot \vec{S}_2 \vec{S}_1 \cdot \vec{v}_2 \hat{n} \cdot \vec{v}_1 - 10 \hat{n} \cdot \vec{S}_2 \hat{n} \cdot \vec{v}_2 \vec{S}_1 \cdot \vec{v}_2 \hat{n} \cdot \vec{v}_1 + \\
& \quad \left. \frac{1}{S_2} \cdot \vec{v}_2 \vec{S}_1 \cdot \vec{v}_2 \hat{n} \cdot \vec{v}_1 + 42 \hat{n} \cdot \vec{S}_1 \hat{n} \cdot \vec{v}_2 \vec{S}_2 \cdot \vec{a}_1 \hat{n} \cdot \vec{v}_1 - \frac{21}{2} \vec{S}_1 \cdot \vec{v}_2 \vec{S}_2 \cdot \vec{a}_1 \hat{n} \cdot \vec{v}_1 - \vec{S}_1 \cdot \vec{v}_2 \vec{S}_2 \cdot \vec{a}_2 \hat{n} \cdot \vec{v}_1 + \right.
\end{aligned}$$



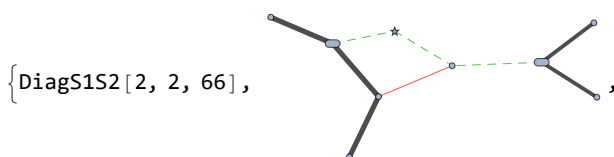

$$G^2 \left( \frac{1}{r} \left( 6 \hat{n} \cdot \vec{S}_2 \vec{S}_1^1 \cdot \vec{a}_2 + 8 \hat{n} \cdot \vec{a}_1 \vec{S}_1^1 \cdot \vec{S}_2 - 12 \hat{n} \cdot \vec{a}_2 \vec{S}_1^1 \cdot \vec{S}_2 - 6 \hat{n} \cdot \vec{v}_2 \vec{S}_1^1 \cdot \vec{S}_2 + 12 \hat{n} \cdot \vec{S}_2 \vec{S}_1^1 \cdot \vec{a}_2 - 6 \hat{n} \cdot \vec{a}_2 \vec{S}_1^1 \cdot \vec{S}_2 + \right. \right. \\ \left. \left. 6 \hat{n} \cdot \vec{S}_2 \vec{S}_1^1 \cdot \vec{v}_2 + 4 \hat{n} \cdot \vec{v}_1 \vec{S}_1^1 \cdot \vec{S}_2 - 4 \hat{n} \cdot \vec{S}_1^1 \vec{S}_2 \cdot \vec{a}_1 - 8 \hat{n} \cdot \vec{S}_1^1 \vec{S}_2 \cdot \vec{a}_1 - 4 \hat{n} \cdot \vec{S}_1^1 \vec{S}_2 \cdot \vec{v}_1 + 4 \hat{n} \cdot \vec{a}_1 \vec{S}_1^1 \cdot \vec{S}_2 \right) + \frac{1}{r^2} \right. \\ \left. \left( -7 \vec{S}_1^1 \cdot \vec{S}_2 (\hat{n} \cdot \vec{v}_1)^2 + 6 \hat{n} \cdot \vec{v}_2 \vec{S}_1^1 \cdot \vec{S}_2 \hat{n} \cdot \vec{v}_1 - 6 \hat{n} \cdot \vec{S}_2 \vec{S}_1^1 \cdot \vec{a}_2 \hat{n} \cdot \vec{v}_1 + 6 \hat{n} \cdot \vec{a}_2 \vec{S}_1^1 \cdot \vec{S}_2 \hat{n} \cdot \vec{v}_1 - 6 \hat{n} \cdot \vec{S}_2 \vec{S}_1^1 \cdot \vec{v}_2 \hat{n} \cdot \vec{v}_1 + \right. \right.$$





$$4 \hat{n} \times \vec{S_1} \cdot \vec{v_1} \hat{n} \times \vec{S_2} \cdot \vec{v_2} \vec{v_2} \cdot \vec{v_2} - \frac{3}{4} \vec{S_1} \cdot \vec{v_2} \vec{S_2} \cdot \vec{v_1} \vec{v_2} \cdot \vec{v_2} + \vec{S_1} \cdot \vec{S_2} \vec{v_1} \cdot \vec{v_1} \vec{v_2} \cdot \vec{v_2} - \frac{3}{4} \vec{S_1} \cdot \vec{S_2} \vec{v_1} \cdot \vec{v_2} \vec{v_2} \cdot \vec{v_2} \Bigg) \Bigg) m_1 \Bigg\}$$

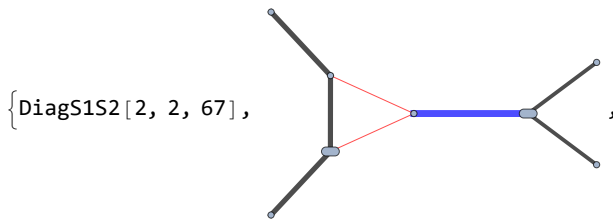

$$G^2 \left( \frac{1}{r^3} \left( -2 \hat{n} \times \vec{S}_2 \cdot \vec{v}_2 \vec{S}_1 \times \vec{v}_1 \cdot \vec{a}_1 + \hat{n} \times \vec{S}_2 \cdot \vec{v}_2 \vec{S}_1 \times \vec{v}_1 \cdot \vec{a}_2 + \frac{3}{2} \hat{n} \times \vec{S}_2 \cdot \vec{v}_2 \vec{S}_1 \times \vec{v}_1 \cdot \vec{v}_2 + \right. \right. \\ 2 \hat{n} \times \vec{S}_2 \cdot \vec{a}_2 \vec{S}_1 \times \vec{v}_1 \cdot \vec{v}_2 - 2 \hat{n} \times \vec{S}_1 \cdot \vec{v}_1 \vec{S}_2 \times \vec{v}_1 \cdot \vec{v}_2 - 2 \hat{n} \times \vec{S}_1 \cdot \vec{a}_1 \vec{S}_2 \times \vec{v}_1 \cdot \vec{v}_2 - 2 \hat{n} \times \vec{S}_1 \cdot \vec{v}_1 \vec{S}_2 \times \vec{v}_2 \cdot \vec{a}_2 - \\ 4 \hat{n} \times \vec{S}_1 \cdot \vec{v}_1 \hat{n} \times \vec{S}_2 \cdot \vec{v}_2 \hat{n} \cdot \vec{a}_2 - 8 \hat{n} \times \vec{S}_1 \cdot \vec{v}_1 \hat{n} \times \vec{S}_2 \cdot \vec{v}_2 \hat{n} \cdot \vec{v}_1 - 8 \hat{n} \times \vec{S}_1 \cdot \vec{a}_1 \hat{n} \times \vec{S}_2 \cdot \vec{v}_2 \hat{n} \cdot \vec{v}_1 - \\ 6 \hat{n} \times \vec{S}_2 \cdot \vec{v}_2 \hat{n} \times \vec{S}_1 \cdot \vec{v}_1 \hat{n} \cdot \vec{v}_2 - 8 \hat{n} \times \vec{S}_1 \cdot \vec{v}_1 \hat{n} \times \vec{S}_2 \cdot \vec{a}_2 \hat{n} \cdot \vec{v}_2 + 2 \hat{n} \cdot \vec{v}_1 \vec{a}_1 \cdot \vec{v}_2 \vec{S}_1 \cdot \vec{S}_2 - \frac{3}{2} \hat{n} \cdot \vec{v}_2 \vec{S}_2 \cdot \vec{v}_1 \vec{S}_1 \cdot \vec{v}_2 - \\ 2 \hat{n} \cdot \vec{v}_1 \vec{S}_1 \cdot \vec{v}_2 \vec{S}_2 \cdot \vec{a}_1 - 2 \hat{n} \cdot \vec{v}_1 \vec{S}_1 \cdot \vec{v}_2 \vec{S}_2 \cdot \vec{v}_1 - 2 \hat{n} \cdot \vec{v}_2 \vec{S}_1 \cdot \vec{a}_2 \vec{S}_2 \cdot \vec{v}_1 - \hat{n} \cdot \vec{a}_2 \vec{S}_1 \cdot \vec{v}_2 \vec{S}_2 \cdot \vec{v}_1 + \\ \left. \left. 2 \hat{n} \cdot \vec{v}_2 \vec{S}_1 \cdot \vec{S}_2 \vec{v}_1 \cdot \vec{a}_2 + 2 \hat{n} \cdot \vec{v}_1 \vec{S}_1 \cdot \vec{S}_2 \vec{v}_1 \cdot \vec{v}_2 + \frac{3}{2} \hat{n} \cdot \vec{v}_2 \vec{S}_1 \cdot \vec{S}_2 \vec{v}_1 \cdot \vec{v}_2 + \hat{n} \cdot \vec{a}_2 \vec{S}_1 \cdot \vec{S}_2 \vec{v}_1 \cdot \vec{v}_2 \right) + \frac{1}{r^4} \right. \\ \left. \left( 24 \hat{n} \times \vec{S}_1 \cdot \vec{v}_1 \hat{n} \times \vec{S}_2 \cdot \vec{v}_2 (\hat{n} \cdot \vec{v}_1)^2 + 4 \vec{S}_1 \cdot \vec{v}_2 \vec{S}_2 \cdot \vec{v}_1 (\hat{n} \cdot \vec{v}_1)^2 - 4 \vec{S}_1 \cdot \vec{S}_2 \vec{v}_1 \cdot \vec{v}_2 (\hat{n} \cdot \vec{v}_1)^2 + 8 \hat{n} \times \vec{S}_1 \cdot \vec{v}_1 \right. \right. \\ \vec{S}_2 \times \vec{v}_1 \cdot \vec{v}_2 \hat{n} \cdot \vec{v}_1 - 24 \hat{n} \times \vec{S}_1 \cdot \vec{v}_1 \hat{n} \times \vec{S}_2 \cdot \vec{v}_2 (\hat{n} \cdot \vec{v}_2)^2 + 8 \hat{n} \times \vec{S}_2 \cdot \vec{v}_2 \vec{S}_1 \times \vec{v}_1 \cdot \vec{v}_2 \hat{n} \cdot \vec{v}_2 - 4 (\hat{n} \cdot \vec{v}_2)^2 \vec{S}_1 \cdot \vec{v}_2 \vec{S}_2 \cdot \vec{v}_1 + \\ \left. \left. 4 (\hat{n} \cdot \vec{v}_2)^2 \vec{S}_1 \cdot \vec{S}_2 \vec{v}_1 \cdot \vec{v}_2 + 6 \hat{n} \times \vec{S}_1 \cdot \vec{v}_1 \hat{n} \times \vec{S}_2 \cdot \vec{v}_2 \vec{v}_2 \cdot \vec{v}_2 + \frac{3}{2} \vec{S}_1 \cdot \vec{v}_2 \vec{S}_2 \cdot \vec{v}_1 \vec{v}_2 \cdot \vec{v}_2 - \frac{3}{2} \vec{S}_1 \cdot \vec{S}_2 \vec{v}_1 \cdot \vec{v}_2 \vec{v}_2 \cdot \vec{v}_2 \right) \right) m_1 \Big\}$$

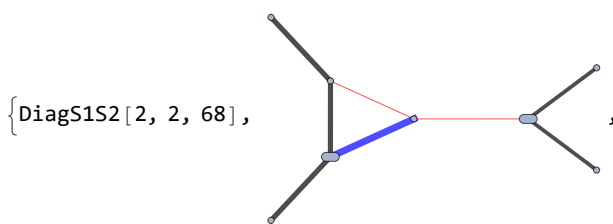

$$\begin{aligned}
G^2 \left( \frac{1}{r^3} \right. & \left( -2 \hat{n} \times \vec{S}_1 \cdot \vec{v}_1 \vec{S}_2 \times \vec{v}_1 \cdot \vec{v}_2 - 8 \hat{n} \times \vec{S}_2 \cdot \vec{v}_2 \vec{S}_1 \times \vec{v}_1 \cdot \vec{a}_1 - 8 \hat{n} \times \vec{S}_1 \cdot \vec{v}_1 \vec{S}_2 \times \vec{a}_1 \cdot \vec{v}_2 - \right. \\
& 2 \hat{n} \times \vec{S}_1 \cdot \vec{v}_1 \vec{S}_2 \times \vec{v}_1 \cdot \vec{a}_2 - 12 \hat{n} \times \vec{S}_1 \cdot \vec{v}_1 \vec{S}_2 \times \vec{v}_1 \cdot \vec{v}_2 - 16 \hat{n} \times \vec{S}_1 \cdot \vec{a}_1 \vec{S}_2 \times \vec{v}_1 \cdot \vec{v}_2 - \hat{n} \times \vec{S}_1 \cdot \vec{v}_1 \vec{S}_2 \times \vec{v}_2 \cdot \vec{a}_2 - \\
& 32 \hat{n} \times \vec{S}_1 \cdot \vec{v}_1 \hat{n} \times \vec{S}_2 \cdot \vec{v}_2 \hat{n} \cdot \vec{a}_1 - 8 \hat{n} \times \vec{S}_2 \cdot \vec{v}_2 \hat{n} \times \vec{S}_1 \cdot \vec{v}_1 \hat{n} \cdot \vec{v}_1 - 8 \hat{n} \times \vec{S}_1 \cdot \vec{v}_1 \hat{n} \times \vec{S}_2 \cdot \vec{a}_2 \hat{n} \cdot \vec{v}_1 - \\
& 48 \hat{n} \times \vec{S}_1 \cdot \vec{v}_1 \hat{n} \times \vec{S}_2 \cdot \vec{v}_2 \hat{n} \cdot \vec{v}_1 - 64 \hat{n} \times \vec{S}_1 \cdot \vec{a}_1 \hat{n} \times \vec{S}_2 \cdot \vec{v}_2 \hat{n} \cdot \vec{v}_1 + 16 \hat{n} \cdot \vec{v}_1 \vec{a}_1 \cdot \vec{v}_2 \vec{S}_1 \cdot \vec{S}_2 - 2 \hat{n} \cdot \vec{v}_1 \vec{S}_2 \cdot \vec{v}_1 \vec{S}_1 \cdot \vec{v}_2 - \\
& 16 \hat{n} \cdot \vec{v}_1 \vec{S}_1 \cdot \vec{v}_2 \vec{S}_2 \cdot \vec{a}_1 - 12 \hat{n} \cdot \vec{v}_1 \vec{S}_1 \cdot \vec{v}_2 \vec{S}_2 \cdot \vec{v}_1 - 2 \hat{n} \cdot \vec{v}_1 \vec{S}_1 \cdot \vec{a}_2 \vec{S}_2 \cdot \vec{v}_1 - 8 \hat{n} \cdot \vec{a}_1 \vec{S}_1 \cdot \vec{v}_2 \vec{S}_2 \cdot \vec{v}_1 + \\
& \left. 2 \hat{n} \cdot \vec{v}_1 \vec{S}_1 \cdot \vec{S}_2 \vec{v}_1 \cdot \vec{a}_2 + 12 \hat{n} \cdot \vec{v}_1 \vec{S}_1 \cdot \vec{S}_2 \vec{v}_1 \cdot \vec{v}_2 + 2 \hat{n} \cdot \vec{v}_1 \vec{S}_1 \cdot \vec{S}_2 \vec{v}_1 \cdot \vec{v}_2 + 8 \hat{n} \cdot \vec{a}_1 \vec{S}_1 \cdot \vec{S}_2 \vec{v}_1 \cdot \vec{v}_2 \right) + \\
& \frac{1}{r^4} \left( 48 \hat{n} \times \vec{S}_1 \cdot \vec{v}_1 \hat{n} \times \vec{S}_2 \cdot \vec{v}_2 (\hat{n} \cdot \vec{v}_1)^2 + 8 \vec{S}_1 \cdot \vec{v}_2 \vec{S}_2 \cdot \vec{v}_1 (\hat{n} \cdot \vec{v}_1)^2 - 8 \vec{S}_1 \cdot \vec{S}_2 \vec{v}_1 \cdot \vec{v}_2 (\hat{n} \cdot \vec{v}_1)^2 + \right. \\
& 8 \hat{n} \times \vec{S}_2 \cdot \vec{v}_2 \vec{S}_1 \times \vec{v}_1 \cdot \vec{v}_2 \hat{n} \cdot \vec{v}_1 + 16 \hat{n} \times \vec{S}_1 \cdot \vec{v}_1 \vec{S}_2 \times \vec{v}_1 \cdot \vec{v}_2 \hat{n} \cdot \vec{v}_1 - 48 \hat{n} \times \vec{S}_1 \cdot \vec{v}_1 \hat{n} \times \vec{S}_2 \cdot \vec{v}_2 \hat{n} \cdot \vec{v}_2 \hat{n} \cdot \vec{v}_1 - \\
& 8 \hat{n} \cdot \vec{v}_2 \vec{S}_1 \cdot \vec{v}_2 \vec{S}_2 \cdot \vec{v}_1 \hat{n} \cdot \vec{v}_1 + 8 \hat{n} \cdot \vec{v}_2 \vec{S}_1 \cdot \vec{S}_2 \vec{v}_1 \cdot \vec{v}_2 \hat{n} \cdot \vec{v}_1 - 2 \vec{S}_1 \cdot \vec{S}_2 (\vec{v}_1 \cdot \vec{v}_2)^2 + \\
& 2 \vec{S}_1 \times \vec{v}_1 \cdot \vec{v}_2 \vec{S}_2 \times \vec{v}_1 \cdot \vec{v}_2 - 8 \hat{n} \times \vec{S}_1 \cdot \vec{v}_1 \vec{S}_2 \times \vec{v}_1 \cdot \vec{v}_2 \hat{n} \cdot \vec{v}_2 - 4 \hat{n} \times \vec{S}_1 \cdot \vec{v}_1 \hat{n} \times \vec{S}_2 \cdot \vec{v}_2 \vec{v}_1 \cdot \vec{v}_1 - \\
& \vec{S}_1 \cdot \vec{v}_2 \vec{S}_2 \cdot \vec{v}_1 \vec{v}_1 \cdot \vec{v}_1 + 8 \hat{n} \times \vec{S}_1 \cdot \vec{v}_1 \hat{n} \times \vec{S}_2 \cdot \vec{v}_2 \vec{v}_1 \cdot \vec{v}_2 + 2 \vec{S}_1 \cdot \vec{v}_2 \vec{S}_2 \cdot \vec{v}_1 \vec{v}_1 \cdot \vec{v}_2 + \vec{S}_1 \cdot \vec{S}_2 \vec{v}_1 \cdot \vec{v}_1 \vec{v}_1 \cdot \vec{v}_2 + \\
& \left. 2 \hat{n} \times \vec{S}_1 \cdot \vec{v}_1 \hat{n} \times \vec{S}_2 \cdot \vec{v}_2 \vec{v}_2 \cdot \vec{v}_2 + \frac{1}{2} \vec{S}_1 \cdot \vec{v}_2 \vec{S}_2 \cdot \vec{v}_1 \vec{v}_2 \cdot \vec{v}_2 - \frac{1}{2} \vec{S}_1 \cdot \vec{S}_2 \vec{v}_1 \cdot \vec{v}_2 \vec{v}_2 \cdot \vec{v}_2 \right) \Big) m_1 \Big\}
\end{aligned}$$

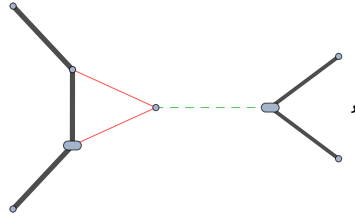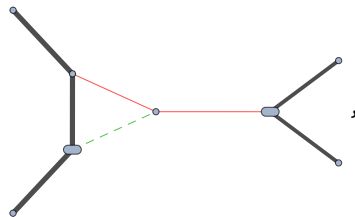

$$G^2 \left( \frac{1}{r^2} \left( 8 \hat{n} \times \vec{S}_1 \cdot \vec{v}_1 \hat{n} \times \vec{S}_2 \cdot \vec{v}_2 + 8 \hat{n} \times \vec{S}_1 \cdot \vec{a}_1 \hat{n} \times \vec{S}_2 \cdot \vec{v}_2 + 8 \hat{n} \times \vec{S}_1 \cdot \vec{v}_1 \hat{n} \times \vec{S}_2 \cdot \vec{a}_2 + \right. \right.$$
  

$$8 \hat{n} \times \vec{S}_1 \cdot \vec{a}_1 \hat{n} \times \vec{S}_2 \cdot \vec{a}_2 + 4 \vec{S}_1 \cdot \vec{v}_2 \vec{S}_2 \cdot \vec{v}_1 - 4 \vec{a}_1 \cdot \vec{v}_2 \vec{S}_1 \cdot \vec{S}_2 - 4 \vec{a}_1 \cdot \vec{a}_2 \vec{S}_1 \cdot \vec{S}_2 +$$
  

$$\left. 4 \vec{S}_2 \cdot \vec{a}_1 \vec{S}_1 \cdot \vec{v}_2 + 4 \vec{S}_1 \cdot \vec{a}_2 \vec{S}_2 \cdot \vec{a}_1 + 4 \vec{S}_1 \cdot \vec{a}_2 \vec{S}_2 \cdot \vec{v}_1 - 4 \vec{S}_1 \cdot \vec{S}_2 \vec{v}_1 \cdot \vec{a}_2 - 4 \vec{S}_1 \cdot \vec{S}_2 \vec{v}_1 \cdot \vec{v}_2 \right) + \frac{1}{r^3}$$
  

$$\left( -8 \hat{n} \times \vec{S}_2 \cdot \vec{v}_2 \vec{S}_1 \times \vec{v}_1 \cdot \vec{v}_2 - 2 \hat{n} \times \vec{S}_1 \cdot \vec{v}_1 \vec{S}_2 \times \vec{v}_1 \cdot \vec{v}_2 - 8 \hat{n} \times \vec{S}_2 \cdot \vec{v}_2 \vec{S}_1 \times \vec{a}_1 \cdot \vec{v}_2 + 8 \hat{n} \times \vec{S}_2 \cdot \vec{v}_2 \vec{S}_1 \times \vec{v}_1 \cdot \vec{a}_1 - \right.$$
  

$$2 \hat{n} \times \vec{S}_1 \cdot \vec{v}_1 \vec{S}_2 \times \vec{v}_1 \cdot \vec{a}_2 + 8 \hat{n} \times \vec{S}_1 \cdot \vec{v}_1 \vec{S}_2 \times \vec{v}_1 \cdot \vec{v}_2 + 8 \hat{n} \times \vec{S}_1 \cdot \vec{a}_1 \vec{S}_2 \times \vec{v}_1 \cdot \vec{v}_2 + \hat{n} \times \vec{S}_1 \cdot \vec{v}_1 \vec{S}_2 \times \vec{v}_2 \cdot \vec{a}_2 -$$
  

$$8 \hat{n} \times \vec{S}_2 \cdot \vec{v}_2 \hat{n} \times \vec{S}_1 \cdot \vec{v}_1 \hat{n} \cdot \vec{v}_1 - 8 \hat{n} \times \vec{S}_1 \cdot \vec{v}_1 \hat{n} \times \vec{S}_2 \cdot \vec{a}_2 \hat{n} \cdot \vec{v}_1 + 32 \hat{n} \times \vec{S}_1 \cdot \vec{v}_1 \hat{n} \times \vec{S}_2 \cdot \vec{v}_2 \hat{n} \cdot \vec{v}_1 +$$
  

$$32 \hat{n} \times \vec{S}_1 \cdot \vec{a}_1 \hat{n} \times \vec{S}_2 \cdot \vec{v}_2 \hat{n} \cdot \vec{v}_1 + 32 \hat{n} \times \vec{S}_1 \cdot \vec{v}_1 \hat{n} \times \vec{S}_2 \cdot \vec{v}_2 \hat{n} \cdot \vec{v}_2 + 32 \hat{n} \times \vec{S}_1 \cdot \vec{a}_1 \hat{n} \times \vec{S}_2 \cdot \vec{v}_2 \hat{n} \cdot \vec{v}_2 -$$
  

$$\left. 8 \hat{n} \cdot \vec{v}_1 \vec{a}_1 \cdot \vec{v}_2 \vec{S}_1 \cdot \vec{S}_2 - 8 \hat{n} \cdot \vec{v}_2 \vec{a}_1 \cdot \vec{v}_2 \vec{S}_1 \cdot \vec{S}_2 - 2 \hat{n} \cdot \vec{v}_1 \vec{S}_2 \cdot \vec{v}_1 \vec{S}_1 \cdot \vec{v}_2 + 8 \hat{n} \cdot \vec{v}_1 \vec{S}_1 \cdot \vec{v}_2 \vec{S}_2 \cdot \vec{a}_1 + \right.$$

$$\begin{aligned}
& 8 \hat{n} \cdot \vec{v}_2 \vec{S}_1 \cdot \vec{v}_2 \vec{S}_2 \cdot \vec{a}_1 + 8 \hat{n} \cdot \vec{v}_1 \vec{S}_1 \cdot \vec{v}_2 \vec{S}_2 \cdot \vec{v}_1 + 8 \hat{n} \cdot \vec{v}_2 \vec{S}_1 \cdot \vec{v}_2 \vec{S}_2 \cdot \vec{v}_1 - 2 \hat{n} \cdot \vec{v}_1 \vec{S}_1 \cdot \vec{a}_2 \vec{S}_2 \cdot \vec{v}_1 + \\
& 2 \hat{n} \cdot \vec{v}_1 \vec{S}_1 \cdot \vec{S}_2 \vec{v}_1 \cdot \vec{a}_2 - 8 \hat{n} \cdot \vec{v}_1 \vec{S}_1 \cdot \vec{S}_2 \vec{v}_1 \cdot \vec{v}_2 - 8 \hat{n} \cdot \vec{v}_2 \vec{S}_1 \cdot \vec{S}_2 \vec{v}_1 \cdot \vec{v}_2 + 2 \hat{n} \cdot \vec{v}_1 \vec{S}_1 \cdot \vec{S}_2 \vec{v}_1 \cdot \vec{v}_2 \Big) + \\
& \frac{1}{r^4} \left( -48 \hat{n} \times \vec{S}_1 \cdot \vec{v}_1 \hat{n} \times \vec{S}_2 \cdot \vec{v}_2 (\hat{n} \cdot \vec{v}_1)^2 - 8 \vec{S}_1 \cdot \vec{v}_2 \vec{S}_2 \cdot \vec{v}_1 (\hat{n} \cdot \vec{v}_1)^2 + 8 \vec{S}_1 \cdot \vec{S}_2 \vec{v}_1 \cdot \vec{v}_2 (\hat{n} \cdot \vec{v}_1)^2 + \right. \\
& 8 \hat{n} \times \vec{S}_2 \cdot \vec{v}_2 \vec{S}_1 \times \vec{v}_1 \cdot \vec{v}_2 \hat{n} \cdot \vec{v}_1 - 16 \hat{n} \times \vec{S}_1 \cdot \vec{v}_1 \vec{S}_2 \times \vec{v}_1 \cdot \vec{v}_2 \hat{n} \cdot \vec{v}_1 - 48 \hat{n} \times \vec{S}_1 \cdot \vec{v}_1 \hat{n} \times \vec{S}_2 \cdot \vec{v}_2 \hat{n} \cdot \vec{v}_2 \hat{n} \cdot \vec{v}_1 - \\
& 8 \hat{n} \cdot \vec{v}_2 \vec{S}_1 \cdot \vec{v}_2 \vec{S}_2 \cdot \vec{v}_1 \hat{n} \cdot \vec{v}_1 + 8 \hat{n} \cdot \vec{v}_2 \vec{S}_1 \cdot \vec{S}_2 \vec{v}_1 \cdot \vec{v}_2 \hat{n} \cdot \vec{v}_1 - 2 \vec{S}_1 \cdot \vec{S}_2 (\vec{v}_1 \cdot \vec{v}_2)^2 + \\
& 2 \vec{S}_1 \times \vec{v}_1 \cdot \vec{v}_2 \vec{S}_2 \times \vec{v}_1 \cdot \vec{v}_2 - 8 \hat{n} \times \vec{S}_1 \cdot \vec{v}_1 \vec{S}_2 \times \vec{v}_1 \cdot \vec{v}_2 \hat{n} \cdot \vec{v}_2 + 4 \hat{n} \times \vec{S}_1 \cdot \vec{v}_1 \hat{n} \times \vec{S}_2 \cdot \vec{v}_2 \vec{v}_1 \cdot \vec{v}_1 + \\
& \vec{S}_1 \cdot \vec{v}_2 \vec{S}_2 \cdot \vec{v}_1 \vec{v}_1 \cdot \vec{v}_1 + 8 \hat{n} \times \vec{S}_1 \cdot \vec{v}_1 \hat{n} \times \vec{S}_2 \cdot \vec{v}_2 \vec{v}_1 \cdot \vec{v}_2 + 2 \vec{S}_1 \cdot \vec{v}_2 \vec{S}_2 \cdot \vec{v}_1 \vec{v}_1 \cdot \vec{v}_2 - \vec{S}_1 \cdot \vec{S}_2 \vec{v}_1 \cdot \vec{v}_1 \vec{v}_1 \cdot \vec{v}_2 - \\
& \left. 2 \hat{n} \times \vec{S}_1 \cdot \vec{v}_1 \hat{n} \times \vec{S}_2 \cdot \vec{v}_2 \vec{v}_2 \cdot \vec{v}_2 - \frac{1}{2} \vec{S}_1 \cdot \vec{v}_2 \vec{S}_2 \cdot \vec{v}_1 \vec{v}_2 \cdot \vec{v}_2 + \frac{1}{2} \vec{S}_1 \cdot \vec{S}_2 \vec{v}_1 \cdot \vec{v}_2 \vec{v}_2 \cdot \vec{v}_2 \right) \Big) m_1 \Big\}
\end{aligned}$$

$$\left\{ \text{DiagS1S2}[3, 1, 1], \right. , \frac{1}{r^5}$$
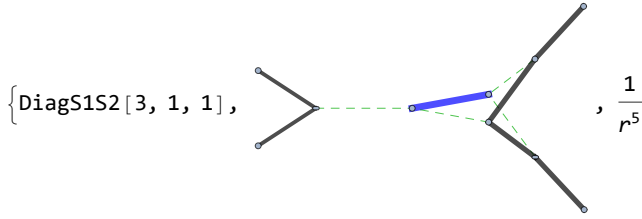

$$\begin{aligned}
& G^3 m_1^2 \left( -\frac{136}{7} \hat{n} \times \vec{S}_1 \cdot \vec{v}_1 \hat{n} \times \vec{S}_2 \cdot \vec{v}_1 - \frac{4}{7} \vec{S}_1 \cdot \vec{S}_2 (\hat{n} \cdot \vec{v}_1)^2 + \frac{4}{7} \hat{n} \cdot \vec{S}_1 \hat{n} \cdot \vec{v}_1 \vec{S}_2 \cdot \vec{v}_1 - \right. \\
& \left. 8 \vec{v}_1 \cdot \vec{v}_1 \hat{n} \cdot \vec{S}_1 \hat{n} \cdot \vec{S}_2 - 4 \vec{S}_1 \cdot \vec{v}_1 \vec{S}_2 \cdot \vec{v}_1 + \frac{44}{5} \vec{S}_1 \cdot \vec{S}_2 \vec{v}_1 \cdot \vec{v}_1 \right) \Big\}
\end{aligned}$$

$$\left\{ \text{DiagS1S2}[3, 1, 2], \right. ,$$
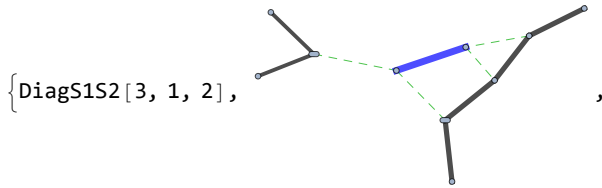

$$\begin{aligned}
& G^3 m_1^2 \left( \frac{1}{r^5 \in_d} \left( -84 \hat{n} \cdot \vec{S}_1 \hat{n} \cdot \vec{S}_2 (\hat{n} \cdot \vec{v}_1)^2 + 12 \vec{S}_1 \cdot \vec{S}_2 (\hat{n} \cdot \vec{v}_1)^2 + 24 \hat{n} \cdot \vec{S}_2 \hat{n} \cdot \vec{v}_1 \vec{S}_1 \cdot \vec{v}_1 + \right. \right. \\
& 24 \hat{n} \cdot \vec{S}_1 \hat{n} \cdot \vec{v}_1 \vec{S}_2 \cdot \vec{v}_1 + 12 \vec{v}_1 \cdot \vec{v}_1 \hat{n} \cdot \vec{S}_1 \hat{n} \cdot \vec{S}_2 - \frac{24}{5} \vec{S}_1 \cdot \vec{v}_1 \vec{S}_2 \cdot \vec{v}_1 - \frac{12}{5} \vec{S}_1 \cdot \vec{S}_2 \vec{v}_1 \cdot \vec{v}_1 \Big) + \\
& \frac{1}{r^5} \log\left(\frac{r}{R_\theta}\right) \left( 252 \hat{n} \cdot \vec{S}_1 \hat{n} \cdot \vec{S}_2 (\hat{n} \cdot \vec{v}_1)^2 - 36 \vec{S}_1 \cdot \vec{S}_2 (\hat{n} \cdot \vec{v}_1)^2 - 72 \hat{n} \cdot \vec{S}_2 \hat{n} \cdot \vec{v}_1 \vec{S}_1 \cdot \vec{v}_1 - \right. \\
& 72 \hat{n} \cdot \vec{S}_1 \hat{n} \cdot \vec{v}_1 \vec{S}_2 \cdot \vec{v}_1 - 36 \vec{v}_1 \cdot \vec{v}_1 \hat{n} \cdot \vec{S}_1 \hat{n} \cdot \vec{S}_2 + \frac{72}{5} \vec{S}_1 \cdot \vec{v}_1 \vec{S}_2 \cdot \vec{v}_1 + \frac{36}{5} \vec{S}_1 \cdot \vec{S}_2 \vec{v}_1 \cdot \vec{v}_1 \Big) + \frac{1}{r^5} \\
& \left( 8 \hat{n} \times \vec{S}_1 \cdot \vec{v}_1 \hat{n} \times \vec{S}_2 \cdot \vec{v}_1 - 148 \hat{n} \cdot \vec{S}_1 \hat{n} \cdot \vec{S}_2 (\hat{n} \cdot \vec{v}_1)^2 + 36 \vec{S}_1 \cdot \vec{S}_2 (\hat{n} \cdot \vec{v}_1)^2 + 32 \hat{n} \cdot \vec{S}_2 \hat{n} \cdot \vec{v}_1 \vec{S}_1 \cdot \vec{v}_1 + \right. \\
& \left. 48 \hat{n} \cdot \vec{S}_1 \hat{n} \cdot \vec{v}_1 \vec{S}_2 \cdot \vec{v}_1 + 28 \vec{v}_1 \cdot \vec{v}_1 \hat{n} \cdot \vec{S}_1 \hat{n} \cdot \vec{S}_2 - \frac{128}{25} \vec{S}_1 \cdot \vec{v}_1 \vec{S}_2 \cdot \vec{v}_1 - \frac{364}{25} \vec{S}_1 \cdot \vec{S}_2 \vec{v}_1 \cdot \vec{v}_1 \right) \Big) \Big\}
\end{aligned}$$

$$\left\{ \text{DiagS1S2}[3, 1, 3], \right. ,$$
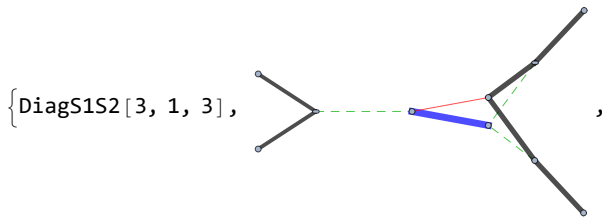

$$G^3 m_1^2 \left( \frac{-5 \hat{n} \cdot \vec{S}_2 \hat{n} \cdot \vec{S}_1 \hat{n} \cdot \vec{v}_1 + \frac{89}{25} \vec{S}_1 \cdot \vec{S}_2 \hat{n} \cdot \vec{v}_1 - \frac{21}{25} \hat{n} \cdot \vec{S}_1 \vec{S}_2 \cdot \vec{v}_1 + \frac{19}{25} \hat{n} \cdot \vec{S}_2 \vec{S}_1 \cdot \vec{v}_1}{r^4} + \frac{1}{r^5} \right)$$

$$\begin{aligned}
& \left( 41 \hat{n} \cdot \vec{S}_1 \hat{n} \cdot \vec{S}_2 (\hat{n} \cdot \vec{v}_1)^2 - \frac{115}{7} \vec{S}_1 \cdot \vec{S}_2 (\hat{n} \cdot \vec{v}_1)^2 - 41 \hat{n} \cdot \vec{S}_1 \hat{n} \cdot \vec{S}_2 \hat{n} \cdot \vec{v}_2 \hat{n} \cdot \vec{v}_1 + 19 \hat{n} \cdot \vec{v}_2 \vec{S}_1 \cdot \vec{S}_2 \hat{n} \cdot \vec{v}_1 - \right. \\
& 10 \hat{n} \cdot \vec{S}_2 \vec{S}_1 \cdot \vec{v}_1 \hat{n} \cdot \vec{v}_1 + 5 \hat{n} \cdot \vec{S}_2 \vec{S}_1 \cdot \vec{v}_2 \hat{n} \cdot \vec{v}_1 - \frac{32}{7} \hat{n} \cdot \vec{S}_1 \vec{S}_2 \cdot \vec{v}_1 \hat{n} \cdot \vec{v}_1 + 5 \hat{n} \cdot \vec{S}_1 \vec{S}_2 \cdot \vec{v}_2 \hat{n} \cdot \vec{v}_1 + \\
& \frac{38}{7} \hat{n} \times \vec{S}_1 \cdot \vec{v}_1 \hat{n} \times \vec{S}_2 \cdot \vec{v}_1 + 5 \hat{n} \cdot \vec{S}_2 \hat{n} \cdot \vec{v}_2 \vec{S}_1 \cdot \vec{v}_1 - 3 \hat{n} \cdot \vec{S}_1 \hat{n} \cdot \vec{v}_2 \vec{S}_2 \cdot \vec{v}_1 + \frac{38}{25} \vec{S}_1 \cdot \vec{v}_1 \vec{S}_2 \cdot \vec{v}_1 + \frac{21}{25} \vec{S}_1 \cdot \vec{v}_2 \vec{S}_2 \cdot \vec{v}_1 - \\
& \frac{19}{25} \vec{S}_1 \cdot \vec{v}_1 \vec{S}_2 \cdot \vec{v}_2 - 5 \hat{n} \cdot \vec{S}_1 \hat{n} \cdot \vec{S}_2 \vec{v}_1 \cdot \vec{v}_1 + \frac{49}{25} \vec{S}_1 \cdot \vec{S}_2 \vec{v}_1 \cdot \vec{v}_1 + 5 \hat{n} \cdot \vec{S}_1 \hat{n} \cdot \vec{S}_2 \vec{v}_1 \cdot \vec{v}_2 - \frac{89}{25} \vec{S}_1 \cdot \vec{S}_2 \vec{v}_1 \cdot \vec{v}_2 \Big) + \\
& \left( \frac{6 \hat{n} \cdot \vec{S}_2 \hat{n} \cdot \vec{S}_1 \hat{n} \cdot \vec{v}_1 - \frac{6}{5} \vec{S}_1 \cdot \vec{S}_2 \hat{n} \cdot \vec{v}_1 - \frac{6}{5} \hat{n} \cdot \vec{S}_1 \vec{S}_2 \cdot \vec{v}_1 - \frac{6}{5} \hat{n} \cdot \vec{S}_2 \vec{S}_1 \cdot \vec{v}_1}{r^4} + \frac{1}{r^5} \right. \\
& \left( -42 \hat{n} \cdot \vec{S}_1 \hat{n} \cdot \vec{S}_2 (\hat{n} \cdot \vec{v}_1)^2 + 6 \vec{S}_1 \cdot \vec{S}_2 (\hat{n} \cdot \vec{v}_1)^2 + 42 \hat{n} \cdot \vec{S}_1 \hat{n} \cdot \vec{S}_2 \hat{n} \cdot \vec{v}_2 \hat{n} \cdot \vec{v}_1 - 6 \hat{n} \cdot \vec{v}_2 \vec{S}_1 \cdot \vec{S}_2 \hat{n} \cdot \vec{v}_1 + \right. \\
& 12 \hat{n} \cdot \vec{S}_2 \vec{S}_1 \cdot \vec{v}_1 \hat{n} \cdot \vec{v}_1 - 6 \hat{n} \cdot \vec{S}_2 \vec{S}_1 \cdot \vec{v}_2 \hat{n} \cdot \vec{v}_1 + 12 \hat{n} \cdot \vec{S}_1 \vec{S}_2 \cdot \vec{v}_1 \hat{n} \cdot \vec{v}_1 - 6 \hat{n} \cdot \vec{S}_1 \vec{S}_2 \cdot \vec{v}_2 \hat{n} \cdot \vec{v}_1 - \\
& 6 \hat{n} \cdot \vec{S}_2 \hat{n} \cdot \vec{v}_2 \vec{S}_1 \cdot \vec{v}_1 - 6 \hat{n} \cdot \vec{S}_1 \hat{n} \cdot \vec{v}_2 \vec{S}_2 \cdot \vec{v}_1 - \frac{12}{5} \vec{S}_1 \cdot \vec{v}_1 \vec{S}_2 \cdot \vec{v}_1 + \frac{6}{5} \vec{S}_1 \cdot \vec{v}_2 \vec{S}_2 \cdot \vec{v}_1 + \frac{6}{5} \vec{S}_1 \cdot \vec{v}_1 \vec{S}_2 \cdot \vec{v}_2 + \\
& \left. 6 \hat{n} \cdot \vec{S}_1 \hat{n} \cdot \vec{S}_2 \vec{v}_1 \cdot \vec{v}_1 - \frac{6}{5} \vec{S}_1 \cdot \vec{S}_2 \vec{v}_1 \cdot \vec{v}_1 - 6 \hat{n} \cdot \vec{S}_1 \hat{n} \cdot \vec{S}_2 \vec{v}_1 \cdot \vec{v}_2 + \frac{6}{5} \vec{S}_1 \cdot \vec{S}_2 \vec{v}_1 \cdot \vec{v}_2 \right) \log \left( \frac{r}{R_\theta} \right) + \\
& \frac{1}{\epsilon_d} \left( \frac{-2 \hat{n} \cdot \vec{S}_2 \hat{n} \cdot \vec{S}_1 \hat{n} \cdot \vec{v}_1 + \frac{2}{5} \vec{S}_1 \cdot \vec{S}_2 \hat{n} \cdot \vec{v}_1 + \frac{2}{5} \hat{n} \cdot \vec{S}_1 \vec{S}_2 \cdot \vec{v}_1 + \frac{2}{5} \hat{n} \cdot \vec{S}_2 \vec{S}_1 \cdot \vec{v}_1}{r^4} + \frac{1}{r^5} \right. \\
& \left( 14 \hat{n} \cdot \vec{S}_1 \hat{n} \cdot \vec{S}_2 (\hat{n} \cdot \vec{v}_1)^2 - 2 \vec{S}_1 \cdot \vec{S}_2 (\hat{n} \cdot \vec{v}_1)^2 - 14 \hat{n} \cdot \vec{S}_1 \hat{n} \cdot \vec{S}_2 \hat{n} \cdot \vec{v}_2 \hat{n} \cdot \vec{v}_1 + 2 \hat{n} \cdot \vec{v}_2 \vec{S}_1 \cdot \vec{S}_2 \hat{n} \cdot \vec{v}_1 - \right. \\
& 4 \hat{n} \cdot \vec{S}_2 \vec{S}_1 \cdot \vec{v}_1 \hat{n} \cdot \vec{v}_1 + 2 \hat{n} \cdot \vec{S}_2 \vec{S}_1 \cdot \vec{v}_2 \hat{n} \cdot \vec{v}_1 - 4 \hat{n} \cdot \vec{S}_1 \vec{S}_2 \cdot \vec{v}_1 \hat{n} \cdot \vec{v}_1 + 2 \hat{n} \cdot \vec{S}_1 \vec{S}_2 \cdot \vec{v}_2 \hat{n} \cdot \vec{v}_1 + \\
& 2 \hat{n} \cdot \vec{S}_2 \hat{n} \cdot \vec{v}_2 \vec{S}_1 \cdot \vec{v}_1 + 2 \hat{n} \cdot \vec{S}_1 \hat{n} \cdot \vec{v}_2 \vec{S}_2 \cdot \vec{v}_1 + \frac{4}{5} \vec{S}_1 \cdot \vec{v}_1 \vec{S}_2 \cdot \vec{v}_1 - \frac{2}{5} \vec{S}_1 \cdot \vec{v}_2 \vec{S}_2 \cdot \vec{v}_1 - \frac{2}{5} \vec{S}_1 \cdot \vec{v}_1 \vec{S}_2 \cdot \vec{v}_2 - \\
& \left. 2 \hat{n} \cdot \vec{S}_1 \hat{n} \cdot \vec{S}_2 \vec{v}_1 \cdot \vec{v}_1 + \frac{2}{5} \vec{S}_1 \cdot \vec{S}_2 \vec{v}_1 \cdot \vec{v}_1 + 2 \hat{n} \cdot \vec{S}_1 \hat{n} \cdot \vec{S}_2 \vec{v}_1 \cdot \vec{v}_2 - \frac{2}{5} \vec{S}_1 \cdot \vec{S}_2 \vec{v}_1 \cdot \vec{v}_2 \right) \Big) \Bigg\}
\end{aligned}$$

{DiagS1S2 [3, 1, 4],

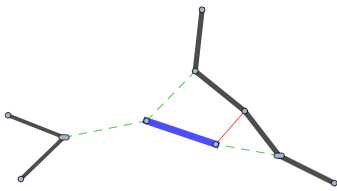

$$\begin{aligned}
& G^3 m_1^2 \left( \frac{2 \hat{n} \cdot \vec{S}_1 \hat{n} \cdot \vec{S}_2 \hat{n} \cdot \vec{v}_1 - \frac{2}{5} \vec{S}_1 \cdot \vec{S}_2 \hat{n} \cdot \vec{v}_1 - \frac{2}{5} \hat{n} \cdot \vec{S}_2 \vec{S}_1 \cdot \vec{v}_1 - \frac{2}{5} \hat{n} \cdot \vec{S}_1 \vec{S}_2 \cdot \vec{v}_1}{r^4 \epsilon_d} + \right. \\
& \frac{10 \hat{n} \times \vec{S}_1 \cdot \vec{v}_1 \hat{n} \times \vec{S}_2 \cdot \vec{v}_1 - 2 \vec{S}_1 \cdot \vec{S}_2 (\hat{n} \cdot \vec{v}_1)^2 + 2 \hat{n} \cdot \vec{S}_1 \hat{n} \cdot \vec{v}_1 \vec{S}_2 \cdot \vec{v}_1 + \frac{8}{5} \vec{S}_1 \cdot \vec{v}_1 \vec{S}_2 \cdot \vec{v}_1 - \frac{8}{5} \vec{S}_1 \cdot \vec{S}_2 \vec{v}_1 \cdot \vec{v}_1}{r^5} + \\
& \left. \log \left( \frac{r}{R_\theta} \right) \left( -6 \hat{n} \cdot \vec{S}_1 \hat{n} \cdot \vec{S}_2 \hat{n} \cdot \vec{v}_1 + \frac{6}{5} \vec{S}_1 \cdot \vec{S}_2 \hat{n} \cdot \vec{v}_1 + \frac{6}{5} \hat{n} \cdot \vec{S}_2 \vec{S}_1 \cdot \vec{v}_1 + \frac{6}{5} \hat{n} \cdot \vec{S}_1 \vec{S}_2 \cdot \vec{v}_1 \right) \right) \Bigg\}
\end{aligned}$$

$$\left. \frac{5 \hat{n} \cdot \vec{S}_1 \hat{n} \cdot \vec{S}_2 \hat{n} \cdot \vec{v}_1 - \frac{9}{25} \vec{S}_1 \cdot \vec{S}_2 \hat{n} \cdot \vec{v}_1 - \frac{19}{25} \hat{n} \cdot \vec{S}_2 \vec{S}_1 \cdot \vec{v}_1 - \frac{59}{25} \hat{n} \cdot \vec{S}_1 \vec{S}_2 \cdot \vec{v}_1}{r^4} \right\}$$

{DiagS1S2 [3, 1, 5],

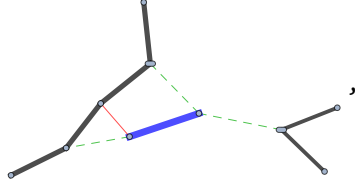

$$G^3 m_1^2 \left( \frac{-60 \hat{n} \cdot \vec{a}_1 \hat{n} \cdot \vec{S}_1 \hat{n} \cdot \vec{S}_2 + 12 \vec{S}_1 \cdot \vec{a}_1 \hat{n} \cdot \vec{S}_2 + 12 \vec{S}_1 \cdot \vec{S}_2 \hat{n} \cdot \vec{a}_1 + 12 \vec{S}_2 \cdot \vec{a}_1 \hat{n} \cdot \vec{S}_1}{r^4 \in_d} + \right. \\ \left. \frac{\log\left(\frac{r}{R_\theta}\right) \left(180 \hat{n} \cdot \vec{a}_1 \hat{n} \cdot \vec{S}_1 \hat{n} \cdot \vec{S}_2 - 36 \vec{S}_1 \cdot \vec{a}_1 \hat{n} \cdot \vec{S}_2 - 36 \vec{S}_1 \cdot \vec{S}_2 \hat{n} \cdot \vec{a}_1 - 36 \vec{S}_2 \cdot \vec{a}_1 \hat{n} \cdot \vec{S}_1\right)}{r^4} + \right. \\ \left. \frac{-176 \hat{n} \cdot \vec{a}_1 \hat{n} \cdot \vec{S}_1 \hat{n} \cdot \vec{S}_2 + 28 \vec{S}_1 \cdot \vec{a}_1 \hat{n} \cdot \vec{S}_2 + 48 \vec{S}_1 \cdot \vec{S}_2 \hat{n} \cdot \vec{a}_1 + 44 \vec{S}_2 \cdot \vec{a}_1 \hat{n} \cdot \vec{S}_1}{r^4} \right\}$$

{DiagS1S2 [3, 1, 6],

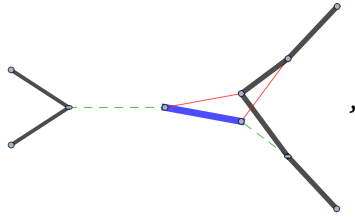

$$G^3 m_1^2 \left( \frac{\frac{11}{3} \vec{S}_1 \cdot \vec{S}_2 - 7 \hat{n} \cdot \vec{S}_1 \hat{n} \cdot \vec{S}_2}{r^3} + \frac{1}{r^4} \left( 11 \hat{n} \cdot \vec{S}_1 \hat{n} \cdot \vec{S}_2 \hat{n} \cdot \vec{v}_1 - \frac{99}{25} \vec{S}_1 \cdot \vec{S}_2 \hat{n} \cdot \vec{v}_1 - 2 \vec{S}_1 \cdot \vec{S}_2 \hat{n} \cdot \vec{v}_1 - 41 \hat{n} \cdot \vec{S}_1 \hat{n} \cdot \vec{S}_2 \hat{n} \cdot \vec{v}_2 + \right. \right. \\ \left. 13 \hat{n} \cdot \vec{v}_2 \vec{S}_1 \cdot \vec{S}_2 - \frac{49}{25} \hat{n} \cdot \vec{S}_2 \vec{S}_1 \cdot \vec{v}_1 + 7 \hat{n} \cdot \vec{S}_2 \vec{S}_1 \cdot \vec{v}_2 + 2 \hat{n} \cdot \vec{S}_1 \vec{S}_2 \cdot \vec{v}_1 - \frac{29}{25} \hat{n} \cdot \vec{S}_1 \vec{S}_2 \cdot \vec{v}_1 + 7 \hat{n} \cdot \vec{S}_1 \vec{S}_2 \cdot \vec{v}_2 \right) + \\ \frac{1}{r^5} \left( 6 \vec{S}_1 \cdot \vec{S}_2 (\hat{n} \cdot \vec{v}_1)^2 - 10 \hat{n} \cdot \vec{v}_2 \vec{S}_1 \cdot \vec{S}_2 \hat{n} \cdot \vec{v}_1 - 6 \hat{n} \cdot \vec{S}_1 \vec{S}_2 \cdot \vec{v}_1 \hat{n} \cdot \vec{v}_1 - 2 \hat{n} \times \vec{S}_1 \cdot \vec{v}_1 \hat{n} \times \vec{S}_2 \cdot \vec{v}_1 + \right. \\ \left. 10 \hat{n} \cdot \vec{S}_1 \hat{n} \cdot \vec{v}_2 \vec{S}_2 \cdot \vec{v}_1 + \frac{4}{5} \vec{S}_1 \cdot \vec{v}_1 \vec{S}_2 \cdot \vec{v}_1 - 2 \vec{S}_1 \cdot \vec{v}_2 \vec{S}_2 \cdot \vec{v}_1 - \frac{4}{5} \vec{S}_1 \cdot \vec{S}_2 \vec{v}_1 \cdot \vec{v}_1 + 2 \vec{S}_1 \cdot \vec{S}_2 \vec{v}_1 \cdot \vec{v}_2 \right) + \\ \left( \frac{6 \hat{n} \cdot \vec{S}_1 \hat{n} \cdot \vec{S}_2 - 2 \vec{S}_1 \cdot \vec{S}_2}{r^3} + \frac{1}{r^4} \left( -6 \hat{n} \cdot \vec{S}_1 \hat{n} \cdot \vec{S}_2 \hat{n} \cdot \vec{v}_1 + \frac{6}{5} \vec{S}_1 \cdot \vec{S}_2 \hat{n} \cdot \vec{v}_1 + 30 \hat{n} \cdot \vec{S}_1 \hat{n} \cdot \vec{S}_2 \hat{n} \cdot \vec{v}_2 - \right. \right. \\ \left. 6 \hat{n} \cdot \vec{v}_2 \vec{S}_1 \cdot \vec{S}_2 + \frac{6}{5} \hat{n} \cdot \vec{S}_2 \vec{S}_1 \cdot \vec{v}_1 - 6 \hat{n} \cdot \vec{S}_2 \vec{S}_1 \cdot \vec{v}_2 + \frac{6}{5} \hat{n} \cdot \vec{S}_1 \vec{S}_2 \cdot \vec{v}_1 - 6 \hat{n} \cdot \vec{S}_1 \vec{S}_2 \cdot \vec{v}_2 \right) \log\left(\frac{r}{R_\theta}\right) + \\ \left. \frac{\frac{2}{3} \vec{S}_1 \cdot \vec{S}_2 - 2 \hat{n} \cdot \vec{S}_1 \hat{n} \cdot \vec{S}_2}{r^3} + \frac{2 \hat{n} \cdot \vec{S}_1 \hat{n} \cdot \vec{S}_2 \hat{n} \cdot \vec{v}_1 - \frac{2}{5} \vec{S}_1 \cdot \vec{S}_2 \hat{n} \cdot \vec{v}_1 - 10 \hat{n} \cdot \vec{S}_1 \hat{n} \cdot \vec{S}_2 \hat{n} \cdot \vec{v}_2 + 2 \hat{n} \cdot \vec{v}_2 \vec{S}_1 \cdot \vec{S}_2 - \frac{2}{5} \hat{n} \cdot \vec{S}_2 \vec{S}_1 \cdot \vec{v}_1 + 2 \hat{n} \cdot \vec{S}_2 \vec{S}_1 \cdot \vec{v}_2 - \frac{2}{5} \hat{n} \cdot \vec{S}_1 \vec{S}_2 \cdot \vec{v}_1 + 2 \hat{n} \cdot \vec{S}_1 \vec{S}_2 \cdot \vec{v}_2}{r^4} \right) \in_d \right\}$$



{DiagS1S2 [3, 1, 7],

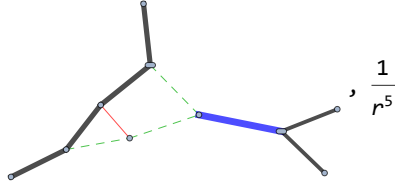

$$G^3 m_1^2 \left( -8 \hat{n} \times \vec{S}_1 \cdot \vec{v}_2 \hat{n} \times \vec{S}_2 \cdot \vec{v}_1 + \frac{64}{7} \hat{n} \times \vec{S}_1 \cdot \vec{v}_1 \hat{n} \times \vec{S}_2 \cdot \vec{v}_2 - \frac{64}{7} \vec{S}_1 \cdot \vec{S}_2 \hat{n} \cdot \vec{v}_1 \hat{n} \cdot \vec{v}_2 + \right. \\ \left. \frac{64}{7} \hat{n} \cdot \vec{S}_1 \hat{n} \cdot \vec{v}_2 \vec{S}_2 \cdot \vec{v}_1 + 8 \vec{v}_1 \cdot \vec{v}_2 \hat{n} \cdot \vec{S}_1 \hat{n} \cdot \vec{S}_2 - \frac{8}{5} \vec{S}_1 \cdot \vec{v}_1 \vec{S}_2 \cdot \vec{v}_2 - \frac{16}{5} \vec{S}_1 \cdot \vec{S}_2 \vec{v}_1 \cdot \vec{v}_2 \right) \Bigg\}$$

{DiagS1S2 [3, 1, 8],

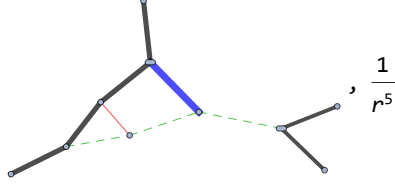

$$G^3 m_1^2 \left( -40 \hat{n} \times \vec{S}_1 \cdot \vec{v}_1 \hat{n} \times \vec{S}_2 \cdot \vec{v}_1 - 8 \vec{S}_1 \cdot \vec{S}_2 (\hat{n} \cdot \vec{v}_1)^2 + 8 \hat{n} \cdot \vec{S}_1 \hat{n} \cdot \vec{v}_1 \vec{S}_2 \cdot \vec{v}_1 - \right. \\ \left. 32 \vec{v}_1 \cdot \vec{v}_1 \hat{n} \cdot \vec{S}_1 \hat{n} \cdot \vec{S}_2 - \frac{48}{5} \vec{S}_1 \cdot \vec{v}_1 \vec{S}_2 \cdot \vec{v}_1 + \frac{144}{5} \vec{S}_1 \cdot \vec{S}_2 \vec{v}_1 \cdot \vec{v}_1 \right) \Bigg\}$$

{DiagS1S2 [3, 1, 9],

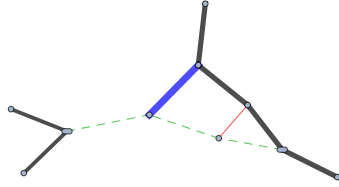

$$G^3 m_1^2 \left( \frac{1}{r^5 \in_d} \left( -56 \hat{n} \cdot \vec{S}_1 \hat{n} \cdot \vec{S}_2 (\hat{n} \cdot \vec{v}_1)^2 + 8 \vec{S}_1 \cdot \vec{S}_2 (\hat{n} \cdot \vec{v}_1)^2 + 16 \hat{n} \cdot \vec{S}_2 \hat{n} \cdot \vec{v}_1 \vec{S}_1 \cdot \vec{v}_1 + \right. \right. \\ \left. 16 \hat{n} \cdot \vec{S}_1 \hat{n} \cdot \vec{v}_1 \vec{S}_2 \cdot \vec{v}_1 + 8 \vec{v}_1 \cdot \vec{v}_1 \hat{n} \cdot \vec{S}_1 \hat{n} \cdot \vec{S}_2 - \frac{16}{5} \vec{S}_1 \cdot \vec{v}_1 \vec{S}_2 \cdot \vec{v}_1 - \frac{8}{5} \vec{S}_1 \cdot \vec{S}_2 \vec{v}_1 \cdot \vec{v}_1 \right) + \\ \frac{1}{r^5} \log \left( \frac{r}{R_0} \right) \left( 168 \hat{n} \cdot \vec{S}_1 \hat{n} \cdot \vec{S}_2 (\hat{n} \cdot \vec{v}_1)^2 - 24 \vec{S}_1 \cdot \vec{S}_2 (\hat{n} \cdot \vec{v}_1)^2 - 48 \hat{n} \cdot \vec{S}_2 \hat{n} \cdot \vec{v}_1 \vec{S}_1 \cdot \vec{v}_1 - \right. \\ \left. 48 \hat{n} \cdot \vec{S}_1 \hat{n} \cdot \vec{v}_1 \vec{S}_2 \cdot \vec{v}_1 - 24 \vec{v}_1 \cdot \vec{v}_1 \hat{n} \cdot \vec{S}_1 \hat{n} \cdot \vec{S}_2 + \frac{48}{5} \vec{S}_1 \cdot \vec{v}_1 \vec{S}_2 \cdot \vec{v}_1 + \frac{24}{5} \vec{S}_1 \cdot \vec{S}_2 \vec{v}_1 \cdot \vec{v}_1 \right) + \frac{1}{r^5} \\ \left. \left( 12 \hat{n} \times \vec{S}_1 \cdot \vec{v}_1 \hat{n} \times \vec{S}_2 \cdot \vec{v}_1 - 136 \hat{n} \cdot \vec{S}_1 \hat{n} \cdot \vec{S}_2 (\hat{n} \cdot \vec{v}_1)^2 + 36 \vec{S}_1 \cdot \vec{S}_2 (\hat{n} \cdot \vec{v}_1)^2 + 32 \hat{n} \cdot \vec{S}_2 \hat{n} \cdot \vec{v}_1 \vec{S}_1 \cdot \vec{v}_1 + \right. \right. \\ \left. \left. 36 \hat{n} \cdot \vec{S}_1 \hat{n} \cdot \vec{v}_1 \vec{S}_2 \cdot \vec{v}_1 + 28 \vec{v}_1 \cdot \vec{v}_1 \hat{n} \cdot \vec{S}_1 \hat{n} \cdot \vec{S}_2 - \frac{72}{25} \vec{S}_1 \cdot \vec{v}_1 \vec{S}_2 \cdot \vec{v}_1 - \frac{396}{25} \vec{S}_1 \cdot \vec{S}_2 \vec{v}_1 \cdot \vec{v}_1 \right) \right) \Bigg\}$$

{DiagS1S2 [3, 1, 10],

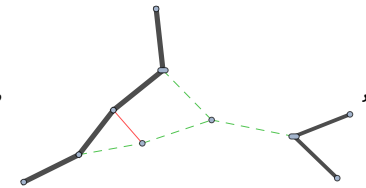

$$G^3 m_1^2 \left( \frac{1}{r^4} \left( 16 \hat{n} \cdot \vec{S}_2 \hat{n} \cdot \vec{S}_1 \hat{n} \cdot \vec{v}_1 - 32 \hat{n} \cdot \vec{S}_1 \hat{n} \cdot \vec{S}_2 \hat{n} \cdot \vec{v}_1 + \frac{88}{5} \vec{S}_1 \cdot \vec{S}_2 \hat{n} \cdot \vec{v}_1 - \frac{184}{25} \vec{S}_1 \cdot \vec{S}_2 \hat{n} \cdot \vec{v}_1 + 4 \hat{n} \cdot \vec{S}_2 \vec{S}_1 \cdot \vec{v}_1 - \right. \right. \\ \left. \frac{84}{25} \hat{n} \cdot \vec{S}_1 \vec{S}_2 \cdot \vec{v}_1 - \frac{8}{5} \hat{n} \cdot \vec{a}_1 \vec{S}_1 \cdot \vec{S}_2 - \frac{44}{25} \hat{n} \cdot \vec{S}_2 \vec{S}_1 \cdot \vec{v}_1 + \frac{8}{5} \hat{n} \cdot \vec{S}_1 \vec{S}_2 \cdot \vec{a}_1 + \frac{12}{5} \hat{n} \cdot \vec{S}_1 \vec{S}_2 \cdot \vec{v}_1 \right) + \frac{1}{r^5} \\ \left. \left( 148 \hat{n} \cdot \vec{S}_1 \hat{n} \cdot \vec{S}_2 (\hat{n} \cdot \vec{v}_1)^2 - \frac{300}{7} \vec{S}_1 \cdot \vec{S}_2 (\hat{n} \cdot \vec{v}_1)^2 + 148 \hat{n} \cdot \vec{S}_1 \hat{n} \cdot \vec{S}_2 \hat{n} \cdot \vec{v}_2 \hat{n} \cdot \vec{v}_1 - 44 \hat{n} \cdot \vec{v}_2 \vec{S}_1 \cdot \vec{S}_2 \hat{n} \cdot \vec{v}_1 - \right. \right. \\ \left. \left. 44 \hat{n} \cdot \vec{v}_2 \vec{S}_1 \cdot \vec{S}_2 \hat{n} \cdot \vec{v}_1 - 44 \hat{n} \cdot \vec{v}_2 \vec{S}_1 \cdot \vec{S}_2 \hat{n} \cdot \vec{v}_1 - 44 \hat{n} \cdot \vec{v}_2 \vec{S}_1 \cdot \vec{S}_2 \hat{n} \cdot \vec{v}_1 \right) \right) \Bigg\}$$

$$\begin{aligned}
& 32 \hat{n} \cdot \vec{S}_2 \vec{S}_1 \cdot \vec{v}_1 \hat{n} \cdot \vec{v}_1 - 16 \hat{n} \cdot \vec{S}_2 \vec{S}_1 \cdot \vec{v}_2 \hat{n} \cdot \vec{v}_1 - \frac{288}{7} \hat{n} \cdot \vec{S}_1 \vec{S}_2 \cdot \vec{v}_1 \hat{n} \cdot \vec{v}_1 - 16 \hat{n} \cdot \vec{S}_1 \vec{S}_2 \cdot \vec{v}_2 \hat{n} \cdot \vec{v}_1 + \\
& \frac{104}{7} \hat{n} \times \vec{S}_1 \cdot \vec{v}_1 \hat{n} \times \vec{S}_2 \cdot \vec{v}_1 - 16 \hat{n} \cdot \vec{S}_2 \hat{n} \cdot \vec{v}_2 \vec{S}_1 \cdot \vec{v}_1 - 24 \hat{n} \cdot \vec{S}_1 \hat{n} \cdot \vec{v}_2 \vec{S}_2 \cdot \vec{v}_1 + \frac{208}{25} \vec{S}_1 \cdot \vec{v}_1 \vec{S}_2 \cdot \vec{v}_1 + \frac{84}{25} \vec{S}_1 \cdot \vec{v}_2 \vec{S}_2 \cdot \vec{v}_1 + \\
& \frac{44}{25} \vec{S}_1 \cdot \vec{v}_1 \vec{S}_2 \cdot \vec{v}_2 - 16 \hat{n} \cdot \vec{S}_1 \hat{n} \cdot \vec{S}_2 \vec{v}_1 \cdot \vec{v}_1 + \frac{104}{25} \vec{S}_1 \cdot \vec{S}_2 \vec{v}_1 \cdot \vec{v}_1 - 16 \hat{n} \cdot \vec{S}_1 \hat{n} \cdot \vec{S}_2 \vec{v}_1 \cdot \vec{v}_2 + \frac{184}{25} \vec{S}_1 \cdot \vec{S}_2 \vec{v}_1 \cdot \vec{v}_2 \Big) + \\
& \left( \frac{1}{r^4} \left( -36 \hat{n} \cdot \vec{S}_2 \hat{n} \cdot \vec{S}_1 \hat{n} \cdot \vec{v}_1 + 60 \hat{n} \cdot \vec{S}_1 \hat{n} \cdot \vec{S}_2 \hat{n} \cdot \vec{v}_1 - 12 \vec{S}_1 \cdot \vec{S}_2 \hat{n} \cdot \vec{v}_1 + \frac{36}{5} \vec{S}_1 \cdot \vec{S}_2 \hat{n} \cdot \vec{v}_1 - \right. \right. \\
& \quad \left. \left. 12 \hat{n} \cdot \vec{S}_2 \vec{S}_1 \cdot \vec{v}_1 + \frac{36}{5} \hat{n} \cdot \vec{S}_1 \vec{S}_2 \cdot \vec{v}_1 + \frac{36}{5} \hat{n} \cdot \vec{S}_2 \vec{S}_1 \cdot \vec{v}_1 - 12 \hat{n} \cdot \vec{S}_1 \vec{S}_2 \cdot \vec{v}_1 \right) + \frac{1}{r^5} \right. \\
& \quad \left( -252 \hat{n} \cdot \vec{S}_1 \hat{n} \cdot \vec{S}_2 (\hat{n} \cdot \vec{v}_1)^2 + 36 \vec{S}_1 \cdot \vec{S}_2 (\hat{n} \cdot \vec{v}_1)^2 - 252 \hat{n} \cdot \vec{S}_1 \hat{n} \cdot \vec{S}_2 \hat{n} \cdot \vec{v}_2 \hat{n} \cdot \vec{v}_1 + 36 \hat{n} \cdot \vec{v}_2 \vec{S}_1 \cdot \vec{S}_2 \hat{n} \cdot \vec{v}_1 + \right. \\
& \quad 72 \hat{n} \cdot \vec{S}_2 \vec{S}_1 \cdot \vec{v}_1 \hat{n} \cdot \vec{v}_1 + 36 \hat{n} \cdot \vec{S}_2 \vec{S}_1 \cdot \vec{v}_2 \hat{n} \cdot \vec{v}_1 + 72 \hat{n} \cdot \vec{S}_1 \vec{S}_2 \cdot \vec{v}_1 \hat{n} \cdot \vec{v}_1 + 36 \hat{n} \cdot \vec{S}_1 \vec{S}_2 \cdot \vec{v}_2 \hat{n} \cdot \vec{v}_1 + \\
& \quad 36 \hat{n} \cdot \vec{S}_2 \hat{n} \cdot \vec{v}_2 \vec{S}_1 \cdot \vec{v}_1 + 36 \hat{n} \cdot \vec{S}_1 \hat{n} \cdot \vec{v}_2 \vec{S}_2 \cdot \vec{v}_1 - \frac{72}{5} \vec{S}_1 \cdot \vec{v}_1 \vec{S}_2 \cdot \vec{v}_1 - \frac{36}{5} \vec{S}_1 \cdot \vec{v}_2 \vec{S}_2 \cdot \vec{v}_1 - \frac{36}{5} \vec{S}_1 \cdot \vec{v}_1 \vec{S}_2 \cdot \vec{v}_2 + \\
& \quad \left. \left. 36 \hat{n} \cdot \vec{S}_1 \hat{n} \cdot \vec{S}_2 \vec{v}_1 \cdot \vec{v}_1 - \frac{36}{5} \vec{S}_1 \cdot \vec{S}_2 \vec{v}_1 \cdot \vec{v}_1 + 36 \hat{n} \cdot \vec{S}_1 \hat{n} \cdot \vec{S}_2 \vec{v}_1 \cdot \vec{v}_2 - \frac{36}{5} \vec{S}_1 \cdot \vec{S}_2 \vec{v}_1 \cdot \vec{v}_2 \right) \right) \log \left( \frac{r}{R_0} \right) + \\
& \frac{1}{\epsilon_d} \left( \frac{1}{r^4} \left( 12 \hat{n} \cdot \vec{S}_2 \hat{n} \cdot \vec{S}_1 \hat{n} \cdot \vec{v}_1 - 20 \hat{n} \cdot \vec{S}_1 \hat{n} \cdot \vec{S}_2 \hat{n} \cdot \vec{v}_1 + 4 \vec{S}_1 \cdot \vec{S}_2 \hat{n} \cdot \vec{v}_1 - \frac{12}{5} \vec{S}_1 \cdot \vec{S}_2 \hat{n} \cdot \vec{v}_1 + \right. \right. \\
& \quad \left. \left. 4 \hat{n} \cdot \vec{S}_2 \vec{S}_1 \cdot \vec{v}_1 - \frac{12}{5} \hat{n} \cdot \vec{S}_1 \vec{S}_2 \cdot \vec{v}_1 - \frac{12}{5} \hat{n} \cdot \vec{S}_2 \vec{S}_1 \cdot \vec{v}_1 + 4 \hat{n} \cdot \vec{S}_1 \vec{S}_2 \cdot \vec{v}_1 \right) + \frac{1}{r^5} \right. \\
& \quad \left( 84 \hat{n} \cdot \vec{S}_1 \hat{n} \cdot \vec{S}_2 (\hat{n} \cdot \vec{v}_1)^2 - 12 \vec{S}_1 \cdot \vec{S}_2 (\hat{n} \cdot \vec{v}_1)^2 + 84 \hat{n} \cdot \vec{S}_1 \hat{n} \cdot \vec{S}_2 \hat{n} \cdot \vec{v}_2 \hat{n} \cdot \vec{v}_1 - 12 \hat{n} \cdot \vec{v}_2 \vec{S}_1 \cdot \vec{S}_2 \hat{n} \cdot \vec{v}_1 - \right. \\
& \quad 24 \hat{n} \cdot \vec{S}_2 \vec{S}_1 \cdot \vec{v}_1 \hat{n} \cdot \vec{v}_1 - 12 \hat{n} \cdot \vec{S}_2 \vec{S}_1 \cdot \vec{v}_2 \hat{n} \cdot \vec{v}_1 - 24 \hat{n} \cdot \vec{S}_1 \vec{S}_2 \cdot \vec{v}_1 \hat{n} \cdot \vec{v}_1 - 12 \hat{n} \cdot \vec{S}_1 \vec{S}_2 \cdot \vec{v}_2 \hat{n} \cdot \vec{v}_1 - \\
& \quad 12 \hat{n} \cdot \vec{S}_2 \hat{n} \cdot \vec{v}_2 \vec{S}_1 \cdot \vec{v}_1 - 12 \hat{n} \cdot \vec{S}_1 \hat{n} \cdot \vec{v}_2 \vec{S}_2 \cdot \vec{v}_1 + \frac{24}{5} \vec{S}_1 \cdot \vec{v}_1 \vec{S}_2 \cdot \vec{v}_1 + \frac{12}{5} \vec{S}_1 \cdot \vec{v}_2 \vec{S}_2 \cdot \vec{v}_1 + \frac{12}{5} \vec{S}_1 \cdot \vec{v}_1 \vec{S}_2 \cdot \vec{v}_2 - \\
& \quad \left. \left. 12 \hat{n} \cdot \vec{S}_1 \hat{n} \cdot \vec{S}_2 \vec{v}_1 \cdot \vec{v}_1 + \frac{12}{5} \vec{S}_1 \cdot \vec{S}_2 \vec{v}_1 \cdot \vec{v}_1 - 12 \hat{n} \cdot \vec{S}_1 \hat{n} \cdot \vec{S}_2 \vec{v}_1 \cdot \vec{v}_2 + \frac{12}{5} \vec{S}_1 \cdot \vec{S}_2 \vec{v}_1 \cdot \vec{v}_2 \right) \right) \Big) \Big\}
\end{aligned}$$

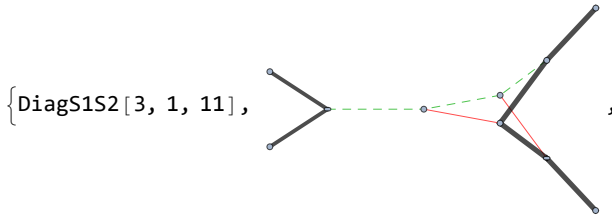

$$\frac{G^3 m_1^2 \left( 104 \hat{n} \times \vec{S}_1 \cdot \vec{v}_1 \hat{n} \times \vec{S}_2 \cdot \vec{v}_1 + 40 \vec{S}_1 \cdot \vec{S}_2 (\hat{n} \cdot \vec{v}_1)^2 - 40 \hat{n} \cdot \vec{S}_1 \hat{n} \cdot \vec{v}_1 \vec{S}_2 \cdot \vec{v}_1 + \frac{144}{5} \vec{S}_1 \cdot \vec{v}_1 \vec{S}_2 \cdot \vec{v}_1 - \frac{144}{5} \vec{S}_1 \cdot \vec{S}_2 \vec{v}_1 \cdot \vec{v}_1 \right)}{r^5} \Big\}$$

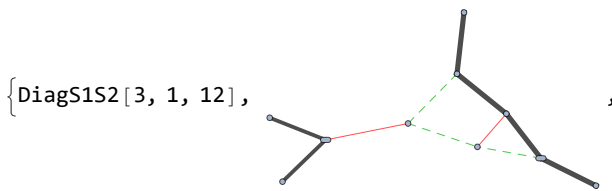

$$\frac{G^3 m_1^2 \left( -16 \hat{n} \times \vec{S}_1 \cdot \vec{v}_1 \hat{n} \times \vec{S}_2 \cdot \vec{v}_2 - \frac{16}{5} \vec{S}_1 \cdot \vec{v}_2 \vec{S}_2 \cdot \vec{v}_1 + \frac{16}{5} \vec{S}_1 \cdot \vec{S}_2 \vec{v}_1 \cdot \vec{v}_2 \right)}{r^5} \Big\}$$

{DiagS1S2[3, 1, 13],

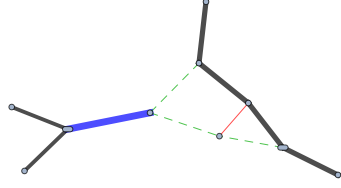

,  $\frac{1}{r^5}$

$$G^3 m_1^2 \left( -4 \hat{n} \times \vec{S}_1 \cdot \vec{v}_2 \hat{n} \times \vec{S}_2 \cdot \vec{v}_1 + \frac{40}{7} \hat{n} \times \vec{S}_1 \cdot \vec{v}_1 \hat{n} \times \vec{S}_2 \cdot \vec{v}_2 - \frac{12}{7} \vec{S}_1 \cdot \vec{S}_2 \hat{n} \cdot \vec{v}_1 \hat{n} \cdot \vec{v}_2 + \right. \\ \left. \frac{12}{7} \hat{n} \cdot \vec{S}_1 \hat{n} \cdot \vec{v}_2 \vec{S}_2 \cdot \vec{v}_1 + 4 \vec{v}_1 \cdot \vec{v}_2 \hat{n} \cdot \vec{S}_1 \hat{n} \cdot \vec{S}_2 + \frac{4}{5} \vec{S}_1 \cdot \vec{v}_2 \vec{S}_2 \cdot \vec{v}_1 - \frac{4}{5} \vec{S}_1 \cdot \vec{v}_1 \vec{S}_2 \cdot \vec{v}_2 - \frac{12}{5} \vec{S}_1 \cdot \vec{S}_2 \vec{v}_1 \cdot \vec{v}_2 \right) \}$$

{DiagS1S2[3, 1, 14],

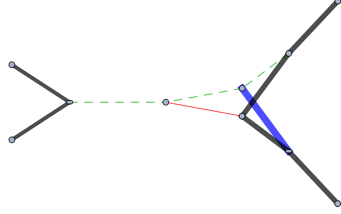

,  $\frac{1}{r^5}$

$$G^3 m_1^2 \left( -54 \hat{n} \times \vec{S}_1 \cdot \vec{v}_1 \hat{n} \times \vec{S}_2 \cdot \vec{v}_1 - 6 \vec{S}_1 \cdot \vec{S}_2 (\hat{n} \cdot \vec{v}_1)^2 + 6 \hat{n} \cdot \vec{S}_1 \hat{n} \cdot \vec{v}_1 \vec{S}_2 \cdot \vec{v}_1 - \right. \\ \left. 36 \vec{v}_1 \cdot \vec{v}_1 \hat{n} \cdot \vec{S}_1 \hat{n} \cdot \vec{S}_2 - 12 \vec{S}_1 \cdot \vec{v}_1 \vec{S}_2 \cdot \vec{v}_1 + \frac{168}{5} \vec{S}_1 \cdot \vec{S}_2 \vec{v}_1 \cdot \vec{v}_1 \right) \}$$

{DiagS1S2[3, 1, 15],

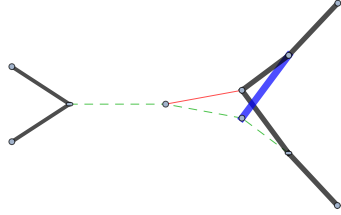

,

$$G^3 m_1^2 \left( \frac{1}{r^{5 \in d}} \left( -96 \hat{n} \cdot \vec{S}_1 \hat{n} \cdot \vec{S}_2 (\hat{n} \cdot \vec{v}_1)^2 + \frac{96}{7} \vec{S}_1 \cdot \vec{S}_2 (\hat{n} \cdot \vec{v}_1)^2 + \frac{192}{7} \hat{n} \cdot \vec{S}_2 \hat{n} \cdot \vec{v}_1 \vec{S}_1 \cdot \vec{v}_1 + \right. \right. \\ \left. \frac{192}{7} \hat{n} \cdot \vec{S}_1 \hat{n} \cdot \vec{v}_1 \vec{S}_2 \cdot \vec{v}_1 + \frac{96}{7} \vec{v}_1 \cdot \vec{v}_1 \hat{n} \cdot \vec{S}_1 \hat{n} \cdot \vec{S}_2 - \frac{192}{35} \vec{S}_1 \cdot \vec{v}_1 \vec{S}_2 \cdot \vec{v}_1 - \frac{96}{35} \vec{S}_1 \cdot \vec{S}_2 \vec{v}_1 \cdot \vec{v}_1 \right) + \\ \frac{1}{r^5} \log \left( \frac{r}{R_0} \right) \left( 288 \hat{n} \cdot \vec{S}_1 \hat{n} \cdot \vec{S}_2 (\hat{n} \cdot \vec{v}_1)^2 - \frac{288}{7} \vec{S}_1 \cdot \vec{S}_2 (\hat{n} \cdot \vec{v}_1)^2 - \frac{576}{7} \hat{n} \cdot \vec{S}_2 \hat{n} \cdot \vec{v}_1 \vec{S}_1 \cdot \vec{v}_1 - \right. \\ \left. \frac{576}{7} \hat{n} \cdot \vec{S}_1 \hat{n} \cdot \vec{v}_1 \vec{S}_2 \cdot \vec{v}_1 - \frac{288}{7} \vec{v}_1 \cdot \vec{v}_1 \hat{n} \cdot \vec{S}_1 \hat{n} \cdot \vec{S}_2 + \frac{576}{35} \vec{S}_1 \cdot \vec{v}_1 \vec{S}_2 \cdot \vec{v}_1 + \frac{288}{35} \vec{S}_1 \cdot \vec{S}_2 \vec{v}_1 \cdot \vec{v}_1 \right) + \frac{1}{r^5} \\ \left( \frac{90}{7} \hat{n} \times \vec{S}_1 \cdot \vec{v}_1 \hat{n} \times \vec{S}_2 \cdot \vec{v}_1 - 32 \hat{n} \cdot \vec{S}_1 \hat{n} \cdot \vec{S}_2 (\hat{n} \cdot \vec{v}_1)^2 + \frac{902}{49} \vec{S}_1 \cdot \vec{S}_2 (\hat{n} \cdot \vec{v}_1)^2 - \frac{128}{49} \hat{n} \cdot \vec{S}_2 \hat{n} \cdot \vec{v}_1 \vec{S}_1 \cdot \vec{v}_1 + \right. \\ \left. \frac{922}{49} \hat{n} \cdot \vec{S}_1 \hat{n} \cdot \vec{v}_1 \vec{S}_2 \cdot \vec{v}_1 + \frac{440}{49} \vec{v}_1 \cdot \vec{v}_1 \hat{n} \cdot \vec{S}_1 \hat{n} \cdot \vec{S}_2 + \frac{2572 \vec{S}_1 \cdot \vec{v}_1 \vec{S}_2 \cdot \vec{v}_1}{1225} - \frac{13204 \vec{S}_1 \cdot \vec{S}_2 \vec{v}_1 \cdot \vec{v}_1}{1225} \right) \right) \}$$

{DiagS1S2[3, 1, 16],

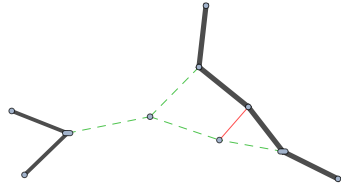

,

$$G^3 m_1^2 \left( \frac{1}{r^4} \left( 16 \hat{n} \cdot \vec{S}_2 \hat{n} \cdot \vec{S}_1 \hat{n} \cdot \vec{v}_1 - 21 \hat{n} \cdot \vec{S}_1 \hat{n} \cdot \vec{S}_2 \hat{n} \cdot \vec{v}_1 + \frac{47}{5} \vec{S}_1 \cdot \vec{S}_2 \hat{n} \cdot \vec{v}_1 - \frac{166}{25} \vec{S}_1 \cdot \vec{S}_2 \hat{n} \cdot \vec{v}_1 + 3 \hat{n} \cdot \vec{S}_2 \vec{S}_1 \cdot \vec{v}_1 - \right. \right.$$

$$\begin{aligned}
& \left( \frac{66}{25} \hat{n} \cdot \vec{S}_1 \vec{S}_2 \cdot \vec{v}_1 - \frac{2}{5} \hat{n} \cdot \vec{a}_1 \vec{S}_1 \cdot \vec{S}_2 - \frac{56}{25} \hat{n} \cdot \vec{S}_2 \vec{S}_1 \cdot \vec{v}_1 + \frac{2}{5} \hat{n} \cdot \vec{S}_1 \vec{S}_2 \cdot \vec{a}_1 + \frac{13}{5} \hat{n} \cdot \vec{S}_1 \vec{S}_2 \cdot \vec{v}_1 \right) + \frac{1}{r^5} \\
& \left( 136 \hat{n} \cdot \vec{S}_1 \hat{n} \cdot \vec{S}_2 (\hat{n} \cdot \vec{v}_1)^2 - \frac{268}{7} \vec{S}_1 \cdot \vec{S}_2 (\hat{n} \cdot \vec{v}_1)^2 + 136 \hat{n} \cdot \vec{S}_1 \hat{n} \cdot \vec{S}_2 \hat{n} \cdot \vec{v}_2 \hat{n} \cdot \vec{v}_1 - 38 \hat{n} \cdot \vec{v}_2 \vec{S}_1 \cdot \vec{S}_2 \hat{n} \cdot \vec{v}_1 - \right. \\
& 32 \hat{n} \cdot \vec{S}_2 \vec{S}_1 \cdot \vec{v}_1 \hat{n} \cdot \vec{v}_1 - 16 \hat{n} \cdot \vec{S}_2 \vec{S}_1 \cdot \vec{v}_2 \hat{n} \cdot \vec{v}_1 - \frac{236}{7} \hat{n} \cdot \vec{S}_1 \vec{S}_2 \cdot \vec{v}_1 \hat{n} \cdot \vec{v}_1 - 16 \hat{n} \cdot \vec{S}_1 \vec{S}_2 \cdot \vec{v}_2 \hat{n} \cdot \vec{v}_1 + \\
& \frac{30}{7} \hat{n} \times \vec{S}_1 \cdot \vec{v}_1 \hat{n} \times \vec{S}_2 \cdot \vec{v}_1 - 16 \hat{n} \cdot \vec{S}_2 \hat{n} \cdot \vec{S}_1 \cdot \vec{v}_2 \vec{S}_1 \cdot \vec{v}_1 - 18 \hat{n} \cdot \vec{S}_1 \hat{n} \cdot \vec{v}_2 \vec{S}_2 \cdot \vec{v}_1 + \frac{142}{25} \vec{S}_1 \cdot \vec{v}_1 \vec{S}_2 \cdot \vec{v}_1 + \frac{66}{25} \vec{S}_1 \cdot \vec{v}_2 \vec{S}_2 \cdot \vec{v}_1 + \\
& \frac{56}{25} \vec{S}_1 \cdot \vec{v}_1 \vec{S}_2 \cdot \vec{v}_2 - 16 \hat{n} \cdot \vec{S}_1 \hat{n} \cdot \vec{S}_2 \vec{v}_1 \cdot \vec{v}_1 + \frac{146}{25} \vec{S}_1 \cdot \vec{S}_2 \vec{v}_1 \cdot \vec{v}_1 - 16 \hat{n} \cdot \vec{S}_1 \hat{n} \cdot \vec{S}_2 \vec{v}_1 \cdot \vec{v}_2 + \frac{166}{25} \vec{S}_1 \cdot \vec{S}_2 \vec{v}_1 \cdot \vec{v}_2 \Big) + \\
& \left( \frac{1}{r^4} \left( -24 \hat{n} \cdot \vec{S}_2 \hat{n} \cdot \vec{S}_1 \hat{n} \cdot \vec{v}_1 + 30 \hat{n} \cdot \vec{S}_1 \hat{n} \cdot \vec{S}_2 \hat{n} \cdot \vec{v}_1 - 6 \vec{S}_1 \cdot \vec{S}_2 \hat{n} \cdot \vec{v}_1 + \frac{24}{5} \vec{S}_1 \cdot \vec{S}_2 \hat{n} \cdot \vec{v}_1 - \right. \right. \\
& 6 \hat{n} \cdot \vec{S}_2 \vec{S}_1 \cdot \vec{v}_1 + \frac{24}{5} \hat{n} \cdot \vec{S}_1 \vec{S}_2 \cdot \vec{v}_1 + \frac{24}{5} \hat{n} \cdot \vec{S}_2 \vec{S}_1 \cdot \vec{v}_1 - 6 \hat{n} \cdot \vec{S}_1 \vec{S}_2 \cdot \vec{v}_1 \Big) + \frac{1}{r^5} \\
& \left( -168 \hat{n} \cdot \vec{S}_1 \hat{n} \cdot \vec{S}_2 (\hat{n} \cdot \vec{v}_1)^2 + 24 \vec{S}_1 \cdot \vec{S}_2 (\hat{n} \cdot \vec{v}_1)^2 - 168 \hat{n} \cdot \vec{S}_1 \hat{n} \cdot \vec{S}_2 \hat{n} \cdot \vec{v}_2 \hat{n} \cdot \vec{v}_1 + 24 \hat{n} \cdot \vec{v}_2 \vec{S}_1 \cdot \vec{S}_2 \hat{n} \cdot \vec{v}_1 + \right. \\
& 48 \hat{n} \cdot \vec{S}_2 \vec{S}_1 \cdot \vec{v}_1 \hat{n} \cdot \vec{v}_1 + 24 \hat{n} \cdot \vec{S}_2 \vec{S}_1 \cdot \vec{v}_2 \hat{n} \cdot \vec{v}_1 + 48 \hat{n} \cdot \vec{S}_1 \vec{S}_2 \cdot \vec{v}_1 \hat{n} \cdot \vec{v}_1 + 24 \hat{n} \cdot \vec{S}_1 \vec{S}_2 \cdot \vec{v}_2 \hat{n} \cdot \vec{v}_1 + \\
& 24 \hat{n} \cdot \vec{S}_2 \hat{n} \cdot \vec{v}_2 \vec{S}_1 \cdot \vec{v}_1 + 24 \hat{n} \cdot \vec{S}_1 \hat{n} \cdot \vec{v}_2 \vec{S}_2 \cdot \vec{v}_1 - \frac{48}{5} \vec{S}_1 \cdot \vec{v}_1 \vec{S}_2 \cdot \vec{v}_1 - \frac{24}{5} \vec{S}_1 \cdot \vec{v}_2 \vec{S}_2 \cdot \vec{v}_1 - \frac{24}{5} \vec{S}_1 \cdot \vec{v}_1 \vec{S}_2 \cdot \vec{v}_2 + \\
& 24 \hat{n} \cdot \vec{S}_1 \hat{n} \cdot \vec{S}_2 \vec{v}_1 \cdot \vec{v}_1 - \frac{24}{5} \vec{S}_1 \cdot \vec{S}_2 \vec{v}_1 \cdot \vec{v}_1 + 24 \hat{n} \cdot \vec{S}_1 \hat{n} \cdot \vec{S}_2 \vec{v}_1 \cdot \vec{v}_2 - \frac{24}{5} \vec{S}_1 \cdot \vec{S}_2 \vec{v}_1 \cdot \vec{v}_2 \Big) \Big) \log \left( \frac{r}{R_0} \right) + \\
& \frac{1}{\epsilon_d} \left( \frac{1}{r^4} \left( 8 \hat{n} \cdot \vec{S}_2 \hat{n} \cdot \vec{S}_1 \hat{n} \cdot \vec{v}_1 - 10 \hat{n} \cdot \vec{S}_1 \hat{n} \cdot \vec{S}_2 \hat{n} \cdot \vec{v}_1 + 2 \vec{S}_1 \cdot \vec{S}_2 \hat{n} \cdot \vec{v}_1 - \frac{8}{5} \vec{S}_1 \cdot \vec{S}_2 \hat{n} \cdot \vec{v}_1 + \right. \right. \\
& 2 \hat{n} \cdot \vec{S}_2 \vec{S}_1 \cdot \vec{v}_1 - \frac{8}{5} \hat{n} \cdot \vec{S}_1 \vec{S}_2 \cdot \vec{v}_1 - \frac{8}{5} \hat{n} \cdot \vec{S}_2 \vec{S}_1 \cdot \vec{v}_1 + 2 \hat{n} \cdot \vec{S}_1 \vec{S}_2 \cdot \vec{v}_1 \Big) + \frac{1}{r^5} \\
& \left( 56 \hat{n} \cdot \vec{S}_1 \hat{n} \cdot \vec{S}_2 (\hat{n} \cdot \vec{v}_1)^2 - 8 \vec{S}_1 \cdot \vec{S}_2 (\hat{n} \cdot \vec{v}_1)^2 + 56 \hat{n} \cdot \vec{S}_1 \hat{n} \cdot \vec{S}_2 \hat{n} \cdot \vec{v}_2 \hat{n} \cdot \vec{v}_1 - 8 \hat{n} \cdot \vec{v}_2 \vec{S}_1 \cdot \vec{S}_2 \hat{n} \cdot \vec{v}_1 - \right. \\
& 16 \hat{n} \cdot \vec{S}_2 \vec{S}_1 \cdot \vec{v}_1 \hat{n} \cdot \vec{v}_1 - 8 \hat{n} \cdot \vec{S}_2 \vec{S}_1 \cdot \vec{v}_2 \hat{n} \cdot \vec{v}_1 - 16 \hat{n} \cdot \vec{S}_1 \vec{S}_2 \cdot \vec{v}_1 \hat{n} \cdot \vec{v}_1 - 8 \hat{n} \cdot \vec{S}_1 \vec{S}_2 \cdot \vec{v}_2 \hat{n} \cdot \vec{v}_1 - \\
& 8 \hat{n} \cdot \vec{S}_2 \hat{n} \cdot \vec{v}_2 \vec{S}_1 \cdot \vec{v}_1 - 8 \hat{n} \cdot \vec{S}_1 \hat{n} \cdot \vec{v}_2 \vec{S}_2 \cdot \vec{v}_1 + \frac{16}{5} \vec{S}_1 \cdot \vec{v}_1 \vec{S}_2 \cdot \vec{v}_1 + \frac{8}{5} \vec{S}_1 \cdot \vec{v}_2 \vec{S}_2 \cdot \vec{v}_1 + \frac{8}{5} \vec{S}_1 \cdot \vec{v}_1 \vec{S}_2 \cdot \vec{v}_2 - \\
& 8 \hat{n} \cdot \vec{S}_1 \hat{n} \cdot \vec{S}_2 \vec{v}_1 \cdot \vec{v}_1 + \frac{8}{5} \vec{S}_1 \cdot \vec{S}_2 \vec{v}_1 \cdot \vec{v}_1 - 8 \hat{n} \cdot \vec{S}_1 \hat{n} \cdot \vec{S}_2 \vec{v}_1 \cdot \vec{v}_2 + \frac{8}{5} \vec{S}_1 \cdot \vec{S}_2 \vec{v}_1 \cdot \vec{v}_2 \Big) \Big) \Big) \Big\}
\end{aligned}$$

{DiagS1S2 [3, 1, 17],

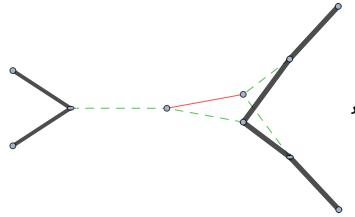

$$\frac{G^3 m_1^2 \left( 24 \hat{n} \times \vec{S}_1 \cdot \vec{v}_1 \hat{n} \times \vec{S}_2 \cdot \vec{v}_1 + 8 \vec{S}_1 \cdot \vec{S}_2 (\hat{n} \cdot \vec{v}_1)^2 - 8 \hat{n} \cdot \vec{S}_1 \hat{n} \cdot \vec{v}_1 \vec{S}_2 \cdot \vec{v}_1 + \frac{32}{5} \vec{S}_1 \cdot \vec{v}_1 \vec{S}_2 \cdot \vec{v}_1 - \frac{32}{5} \vec{S}_1 \cdot \vec{S}_2 \vec{v}_1 \cdot \vec{v}_1 \right)}{r^5} \Big\}$$

{DiagS1S2 [3, 1, 18],

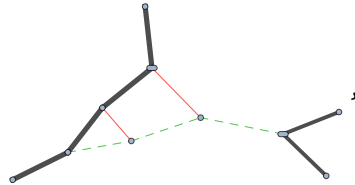

$$\frac{G^3 m_1^2 \left( 96 \hat{n} \times \vec{S}_1 \cdot \vec{v}_1 \hat{n} \times \vec{S}_2 \cdot \vec{v}_1 + 32 \vec{S}_1 \cdot \vec{S}_2 (\hat{n} \cdot \vec{v}_1)^2 - 32 \hat{n} \cdot \vec{S}_1 \hat{n} \cdot \vec{v}_1 \vec{S}_2 \cdot \vec{v}_1 + \frac{128}{5} \vec{S}_1 \cdot \vec{v}_1 \vec{S}_2 \cdot \vec{v}_1 - \frac{128}{5} \vec{S}_1 \cdot \vec{S}_2 \vec{v}_1 \cdot \vec{v}_1 \right)}{r^5} \Big\}$$

{DiagS1S2 [3, 1, 19],

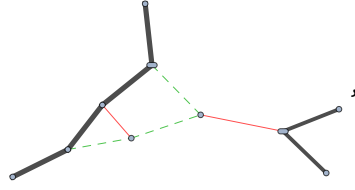

$$\frac{G^3 m_1^2 \left( -32 \hat{n} \times \vec{S}_1 \cdot \vec{v}_1 \hat{n} \times \vec{S}_2 \cdot \vec{v}_2 - \frac{32}{5} \vec{S}_1 \cdot \vec{v}_2 \vec{S}_2 \cdot \vec{v}_1 + \frac{32}{5} \vec{S}_1 \cdot \vec{S}_2 \vec{v}_1 \cdot \vec{v}_2 \right)}{r^5} \}$$

{DiagS1S2 [3, 1, 20],

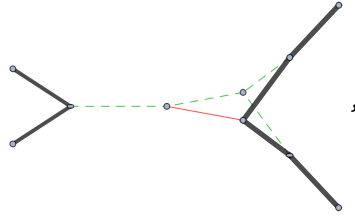

$$\begin{aligned} G^3 m_1^2 \left( \frac{1}{r^4} \left( 3 \hat{n} \cdot \vec{S}_2 \hat{n} \cdot \vec{S}_1 \hat{n} \cdot \vec{v}_1 - 8 \hat{n} \cdot \vec{S}_1 \hat{n} \cdot \vec{S}_2 \hat{n} \cdot \vec{v}_1 + \frac{508}{25} \vec{S}_1 \cdot \vec{S}_2 \hat{n} \cdot \vec{v}_1 - \frac{191}{25} \vec{S}_1 \cdot \vec{S}_2 \hat{n} \cdot \vec{v}_1 - \frac{32}{25} \hat{n} \cdot \vec{S}_2 \vec{S}_1 \cdot \vec{v}_1 - \right. \right. \\ \left. \frac{1}{25} \hat{n} \cdot \vec{S}_1 \vec{S}_2 \cdot \vec{v}_1 - 4 \hat{n} \cdot \vec{S}_1 \vec{S}_2 \cdot \vec{v}_1 + \frac{39}{25} \hat{n} \cdot \vec{S}_2 \vec{S}_1 \cdot \vec{v}_1 + 4 \hat{n} \cdot \vec{S}_1 \vec{S}_2 \cdot \vec{v}_1 - \frac{212}{25} \hat{n} \cdot \vec{S}_1 \vec{S}_2 \cdot \vec{v}_1 \right) + \frac{1}{r^5} \\ \left( -11 \hat{n} \cdot \vec{S}_1 \hat{n} \cdot \vec{S}_2 (\hat{n} \cdot \vec{v}_1)^2 - \frac{1167}{49} \vec{S}_1 \cdot \vec{S}_2 (\hat{n} \cdot \vec{v}_1)^2 + 75 \hat{n} \cdot \vec{S}_1 \hat{n} \cdot \vec{S}_2 \hat{n} \cdot \vec{v}_2 \hat{n} \cdot \vec{v}_1 - 49 \hat{n} \cdot \vec{v}_2 \vec{S}_1 \cdot \vec{S}_2 \hat{n} \cdot \vec{v}_1 + \right. \\ \frac{550}{49} \hat{n} \cdot \vec{S}_2 \vec{S}_1 \cdot \vec{v}_1 \hat{n} \cdot \vec{v}_1 - 3 \hat{n} \cdot \vec{S}_2 \vec{S}_1 \cdot \vec{v}_2 \hat{n} \cdot \vec{v}_1 + \frac{606}{49} \hat{n} \cdot \vec{S}_1 \vec{S}_2 \cdot \vec{v}_1 \hat{n} \cdot \vec{v}_1 - 3 \hat{n} \cdot \vec{S}_1 \vec{S}_2 \cdot \vec{v}_2 \hat{n} \cdot \vec{v}_1 + \\ \frac{240}{7} \hat{n} \cdot \vec{S}_1 \cdot \vec{v}_1 \hat{n} \cdot \vec{S}_2 \cdot \vec{v}_1 - 3 \hat{n} \cdot \vec{S}_2 \hat{n} \cdot \vec{v}_2 \vec{S}_1 \cdot \vec{v}_1 - 11 \hat{n} \cdot \vec{S}_1 \hat{n} \cdot \vec{v}_2 \vec{S}_2 \cdot \vec{v}_1 + \frac{2598 \vec{S}_1 \cdot \vec{v}_1 \vec{S}_2 \cdot \vec{v}_1}{1225} + \frac{1}{25} \vec{S}_1 \cdot \vec{v}_2 \vec{S}_2 \cdot \vec{v}_1 - \\ \left. \frac{39}{25} \vec{S}_1 \cdot \vec{v}_1 \vec{S}_2 \cdot \vec{v}_2 + \frac{443}{49} \hat{n} \cdot \vec{S}_1 \hat{n} \cdot \vec{S}_2 \vec{v}_1 \cdot \vec{v}_1 - \frac{6471 \vec{S}_1 \cdot \vec{S}_2 \vec{v}_1 \cdot \vec{v}_1}{1225} - 3 \hat{n} \cdot \vec{S}_1 \hat{n} \cdot \vec{S}_2 \vec{v}_1 \cdot \vec{v}_2 + \frac{191}{25} \vec{S}_1 \cdot \vec{S}_2 \vec{v}_1 \cdot \vec{v}_2 \right) + \\ \left( \frac{1}{r^4} \left( -54 \hat{n} \cdot \vec{S}_2 \hat{n} \cdot \vec{S}_1 \hat{n} \cdot \vec{v}_1 + 72 \hat{n} \cdot \vec{S}_1 \hat{n} \cdot \vec{S}_2 \hat{n} \cdot \vec{v}_1 - \frac{72}{5} \vec{S}_1 \cdot \vec{S}_2 \hat{n} \cdot \vec{v}_1 + \frac{54}{5} \vec{S}_1 \cdot \vec{S}_2 \hat{n} \cdot \vec{v}_1 - \right. \right. \\ \left. \frac{72}{5} \hat{n} \cdot \vec{S}_2 \vec{S}_1 \cdot \vec{v}_1 + \frac{54}{5} \hat{n} \cdot \vec{S}_1 \vec{S}_2 \cdot \vec{v}_1 + \frac{54}{5} \hat{n} \cdot \vec{S}_2 \vec{S}_1 \cdot \vec{v}_1 - \frac{72}{5} \hat{n} \cdot \vec{S}_1 \vec{S}_2 \cdot \vec{v}_1 \right) + \frac{1}{r^5} \\ \left( -198 \hat{n} \cdot \vec{S}_1 \hat{n} \cdot \vec{S}_2 (\hat{n} \cdot \vec{v}_1)^2 + \frac{198}{7} \vec{S}_1 \cdot \vec{S}_2 (\hat{n} \cdot \vec{v}_1)^2 - 378 \hat{n} \cdot \vec{S}_1 \hat{n} \cdot \vec{S}_2 \hat{n} \cdot \vec{v}_2 \hat{n} \cdot \vec{v}_1 + 54 \hat{n} \cdot \vec{v}_2 \vec{S}_1 \cdot \vec{S}_2 \hat{n} \cdot \vec{v}_1 + \right. \\ \frac{396}{7} \hat{n} \cdot \vec{S}_2 \vec{S}_1 \cdot \vec{v}_1 \hat{n} \cdot \vec{v}_1 + 54 \hat{n} \cdot \vec{S}_2 \vec{S}_1 \cdot \vec{v}_2 \hat{n} \cdot \vec{v}_1 + \frac{396}{7} \hat{n} \cdot \vec{S}_1 \vec{S}_2 \cdot \vec{v}_1 \hat{n} \cdot \vec{v}_1 + 54 \hat{n} \cdot \vec{S}_1 \vec{S}_2 \cdot \vec{v}_2 \hat{n} \cdot \vec{v}_1 + \\ 54 \hat{n} \cdot \vec{S}_2 \hat{n} \cdot \vec{v}_2 \vec{S}_1 \cdot \vec{v}_1 + 54 \hat{n} \cdot \vec{S}_1 \hat{n} \cdot \vec{v}_2 \vec{S}_2 \cdot \vec{v}_1 - \frac{396}{35} \vec{S}_1 \cdot \vec{v}_1 \vec{S}_2 \cdot \vec{v}_1 - \frac{54}{5} \vec{S}_1 \cdot \vec{v}_2 \vec{S}_2 \cdot \vec{v}_1 - \frac{54}{5} \vec{S}_1 \cdot \vec{v}_1 \vec{S}_2 \cdot \vec{v}_2 + \\ \left. \frac{198}{7} \hat{n} \cdot \vec{S}_1 \hat{n} \cdot \vec{S}_2 \vec{v}_1 \cdot \vec{v}_1 - \frac{198}{35} \vec{S}_1 \cdot \vec{S}_2 \vec{v}_1 \cdot \vec{v}_1 + 54 \hat{n} \cdot \vec{S}_1 \hat{n} \cdot \vec{S}_2 \vec{v}_1 \cdot \vec{v}_2 - \frac{54}{5} \vec{S}_1 \cdot \vec{S}_2 \vec{v}_1 \cdot \vec{v}_2 \right) \log \left( \frac{r}{R_\theta} \right) + \\ \frac{1}{\epsilon_d} \left( \frac{1}{r^4} \left( 18 \hat{n} \cdot \vec{S}_2 \hat{n} \cdot \vec{S}_1 \hat{n} \cdot \vec{v}_1 - 24 \hat{n} \cdot \vec{S}_1 \hat{n} \cdot \vec{S}_2 \hat{n} \cdot \vec{v}_1 + \frac{24}{5} \vec{S}_1 \cdot \vec{S}_2 \hat{n} \cdot \vec{v}_1 - \frac{18}{5} \vec{S}_1 \cdot \vec{S}_2 \hat{n} \cdot \vec{v}_1 + \right. \right. \\ \left. \frac{24}{5} \hat{n} \cdot \vec{S}_2 \vec{S}_1 \cdot \vec{v}_1 - \frac{18}{5} \hat{n} \cdot \vec{S}_1 \vec{S}_2 \cdot \vec{v}_1 - \frac{18}{5} \hat{n} \cdot \vec{S}_2 \vec{S}_1 \cdot \vec{v}_1 + \frac{24}{5} \hat{n} \cdot \vec{S}_1 \vec{S}_2 \cdot \vec{v}_1 \right) + \frac{1}{r^5} \\ \left( 66 \hat{n} \cdot \vec{S}_1 \hat{n} \cdot \vec{S}_2 (\hat{n} \cdot \vec{v}_1)^2 - \frac{66}{7} \vec{S}_1 \cdot \vec{S}_2 (\hat{n} \cdot \vec{v}_1)^2 + 126 \hat{n} \cdot \vec{S}_1 \hat{n} \cdot \vec{S}_2 \hat{n} \cdot \vec{v}_2 \hat{n} \cdot \vec{v}_1 - 18 \hat{n} \cdot \vec{v}_2 \vec{S}_1 \cdot \vec{S}_2 \hat{n} \cdot \vec{v}_1 - \right. \\ \left. \frac{132}{7} \hat{n} \cdot \vec{S}_2 \vec{S}_1 \cdot \vec{v}_1 \hat{n} \cdot \vec{v}_1 - 18 \hat{n} \cdot \vec{S}_2 \vec{S}_1 \cdot \vec{v}_2 \hat{n} \cdot \vec{v}_1 - \frac{132}{7} \hat{n} \cdot \vec{S}_1 \vec{S}_2 \cdot \vec{v}_1 \hat{n} \cdot \vec{v}_1 - 18 \hat{n} \cdot \vec{S}_1 \vec{S}_2 \cdot \vec{v}_2 \hat{n} \cdot \vec{v}_1 - \right. \\ \left. 18 \hat{n} \cdot \vec{S}_2 \hat{n} \cdot \vec{v}_2 \vec{S}_1 \cdot \vec{v}_1 - 18 \hat{n} \cdot \vec{S}_1 \hat{n} \cdot \vec{v}_2 \vec{S}_2 \cdot \vec{v}_1 + \frac{132}{35} \vec{S}_1 \cdot \vec{v}_1 \vec{S}_2 \cdot \vec{v}_1 + \frac{18}{5} \vec{S}_1 \cdot \vec{v}_2 \vec{S}_2 \cdot \vec{v}_1 + \frac{18}{5} \vec{S}_1 \cdot \vec{v}_1 \vec{S}_2 \cdot \vec{v}_2 - \right. \end{aligned}$$

$$\left. \left. \left. \frac{66}{7} \hat{n} \cdot \vec{S}_1 \hat{n} \cdot \vec{S}_2 \vec{v}_1 \cdot \vec{v}_1 + \frac{66}{35} \vec{S}_1 \cdot \vec{S}_2 \vec{v}_1 \cdot \vec{v}_1 - 18 \hat{n} \cdot \vec{S}_1 \hat{n} \cdot \vec{S}_2 \vec{v}_1 \cdot \vec{v}_2 + \frac{18}{5} \vec{S}_1 \cdot \vec{S}_2 \vec{v}_1 \cdot \vec{v}_2 \right) \right) \right)$$

$$\left\{ \text{DiagS1S2}[3, 1, 21], \quad \frac{G^3 m_1^2 \left( \frac{48}{5} \vec{S}_1 \cdot \vec{S}_2 \vec{v}_1 \cdot \vec{v}_1 - 16 \vec{v}_1 \cdot \vec{v}_1 \hat{n} \cdot \vec{S}_1 \hat{n} \cdot \vec{S}_2 \right)}{r^5} \right\}$$

$\{\text{DiagS1S2}[3, 1, 22],$

$$G^3 m_1^2 \left( \frac{-2 \hat{n} \cdot \vec{S_1} \hat{n} \cdot \vec{S_2} \hat{n} \cdot \vec{v_2} + \frac{2}{5} \vec{S_1} \cdot \vec{S_2} \hat{n} \cdot \vec{v_2} + \frac{2}{5} \hat{n} \cdot \vec{S_2} \vec{S_1} \cdot \vec{v_2} + \frac{2}{5} \hat{n} \cdot \vec{S_1} \vec{S_2} \cdot \vec{v_2}}{r^4 \in_d} + \right. \\ \left. \frac{2 \vec{S_1} \cdot \vec{S_2} \hat{n} \cdot \vec{v_1} \hat{n} \cdot \vec{v_2} - 2 \hat{n} \cdot \vec{S_1} \hat{n} \cdot \vec{v_2} \vec{S_2} \cdot \vec{v_1} - \frac{2}{5} \vec{S_1} \cdot \vec{S_2} \vec{v_1} \cdot \vec{v_2} + \frac{2}{5} \vec{S_1} \cdot \vec{v_2} \vec{S_2} \cdot \vec{v_1}}{r^5} + \right. \\ \left. \frac{\log\left(\frac{r}{R_0}\right) \left( 6 \hat{n} \cdot \vec{S_1} \hat{n} \cdot \vec{S_2} \hat{n} \cdot \vec{v_2} - \frac{6}{5} \vec{S_1} \cdot \vec{S_2} \hat{n} \cdot \vec{v_2} - \frac{6}{5} \hat{n} \cdot \vec{S_2} \vec{S_1} \cdot \vec{v_2} - \frac{6}{5} \hat{n} \cdot \vec{S_1} \vec{S_2} \cdot \vec{v_2} \right)}{r^4} + \right. \\ \left. \frac{-5 \hat{n} \cdot \vec{S_1} \hat{n} \cdot \vec{S_2} \hat{n} \cdot \vec{v_2} + \frac{49}{25} \vec{S_1} \cdot \vec{S_2} \hat{n} \cdot \vec{v_2} + \frac{19}{25} \hat{n} \cdot \vec{S_2} \vec{S_1} \cdot \vec{v_2} + \frac{19}{25} \hat{n} \cdot \vec{S_1} \vec{S_2} \cdot \vec{v_2}}{r^4} \right\}$$

$\{\text{DiagS1S2}[3, 1, 23],$

$$G^3 m_1^2 \left( \frac{-5 \hat{n} \cdot \vec{S}_2 \hat{n} \cdot \vec{S}_1 \hat{n} \cdot \vec{v}_1 + \frac{217}{25} \vec{S}_1 \cdot \vec{S}_2 \hat{n} \cdot \vec{v}_1 - \frac{113}{25} \hat{n} \cdot \vec{S}_1 \vec{S}_2 \cdot \vec{v}_1 + \frac{7}{25} \hat{n} \cdot \vec{S}_2 \vec{S}_1 \cdot \vec{v}_1}{r^4} + \frac{1}{r^5} \right. \\ \left( 53 \hat{n} \cdot \vec{S}_1 \hat{n} \cdot \vec{S}_2 (\hat{n} \cdot \vec{v}_1)^2 - 49 \vec{S}_1 \cdot \vec{S}_2 (\hat{n} \cdot \vec{v}_1)^2 - 53 \hat{n} \cdot \vec{S}_1 \hat{n} \cdot \vec{S}_2 \hat{n} \cdot \vec{v}_2 \hat{n} \cdot \vec{v}_1 + 47 \hat{n} \cdot \vec{v}_2 \vec{S}_1 \cdot \vec{S}_2 \hat{n} \cdot \vec{v}_1 - \right. \\ 10 \hat{n} \cdot \vec{S}_2 \vec{S}_1 \cdot \vec{v}_1 \hat{n} \cdot \vec{v}_1 + 5 \hat{n} \cdot \vec{S}_2 \vec{S}_1 \cdot \vec{v}_2 \hat{n} \cdot \vec{v}_1 + 16 \hat{n} \cdot \vec{S}_1 \vec{S}_2 \cdot \vec{v}_1 \hat{n} \cdot \vec{v}_1 + 5 \hat{n} \cdot \vec{S}_1 \vec{S}_2 \cdot \vec{v}_2 \hat{n} \cdot \vec{v}_1 + \\ 14 \hat{n} \times \vec{S}_1 \cdot \vec{v}_1 \hat{n} \times \vec{S}_2 \cdot \vec{v}_1 + 5 \hat{n} \cdot \vec{S}_2 \hat{n} \cdot \vec{v}_2 \vec{S}_1 \cdot \vec{v}_1 - 19 \hat{n} \cdot \vec{S}_1 \hat{n} \cdot \vec{v}_2 \vec{S}_2 \cdot \vec{v}_1 - \frac{46}{25} \vec{S}_1 \cdot \vec{v}_1 \vec{S}_2 \cdot \vec{v}_1 + \frac{113}{25} \vec{S}_1 \cdot \vec{v}_2 \vec{S}_2 \cdot \vec{v}_1 - \\ \left. \frac{7}{25} \vec{S}_1 \cdot \vec{v}_1 \vec{S}_2 \cdot \vec{v}_2 - 5 \hat{n} \cdot \vec{S}_1 \hat{n} \cdot \vec{S}_2 \vec{v}_1 \cdot \vec{v}_1 + \frac{157}{25} \vec{S}_1 \cdot \vec{S}_2 \vec{v}_1 \cdot \vec{v}_1 + 5 \hat{n} \cdot \vec{S}_1 \hat{n} \cdot \vec{S}_2 \vec{v}_1 \cdot \vec{v}_2 - \frac{217}{25} \vec{S}_1 \cdot \vec{S}_2 \vec{v}_1 \cdot \vec{v}_2 \right) + \\ \left. \left( \frac{18 \hat{n} \cdot \vec{S}_2 \hat{n} \cdot \vec{S}_1 \hat{n} \cdot \vec{v}_1 - \frac{18}{5} \vec{S}_1 \cdot \vec{S}_2 \hat{n} \cdot \vec{v}_1 - \frac{18}{5} \hat{n} \cdot \vec{S}_1 \vec{S}_2 \cdot \vec{v}_1 - \frac{18}{5} \hat{n} \cdot \vec{S}_2 \vec{S}_1 \cdot \vec{v}_1}{r^4} + \frac{1}{r^5} \right) \right)$$

$$\begin{aligned}
& \left( -126 \hat{n} \cdot \vec{S}_1 \hat{n} \cdot \vec{S}_2 (\hat{n} \cdot \vec{v}_1)^2 + 18 \vec{S}_1 \cdot \vec{S}_2 (\hat{n} \cdot \vec{v}_1)^2 + 126 \hat{n} \cdot \vec{S}_1 \hat{n} \cdot \vec{S}_2 \hat{n} \cdot \vec{v}_2 \hat{n} \cdot \vec{v}_1 - 18 \hat{n} \cdot \vec{v}_2 \vec{S}_1 \cdot \vec{S}_2 \hat{n} \cdot \vec{v}_1 + \right. \\
& 36 \hat{n} \cdot \vec{S}_2 \vec{S}_1 \cdot \vec{v}_1 \hat{n} \cdot \vec{v}_1 - 18 \hat{n} \cdot \vec{S}_2 \vec{S}_1 \cdot \vec{v}_2 \hat{n} \cdot \vec{v}_1 + 36 \hat{n} \cdot \vec{S}_1 \vec{S}_2 \cdot \vec{v}_1 \hat{n} \cdot \vec{v}_1 - 18 \hat{n} \cdot \vec{S}_1 \vec{S}_2 \cdot \vec{v}_2 \hat{n} \cdot \vec{v}_1 - \\
& 18 \hat{n} \cdot \vec{S}_2 \hat{n} \cdot \vec{v}_2 \vec{S}_1 \cdot \vec{v}_1 - 18 \hat{n} \cdot \vec{S}_1 \hat{n} \cdot \vec{v}_2 \vec{S}_2 \cdot \vec{v}_1 - \frac{36}{5} \vec{S}_1 \cdot \vec{v}_1 \vec{S}_2 \cdot \vec{v}_1 + \frac{18}{5} \vec{S}_1 \cdot \vec{v}_2 \vec{S}_2 \cdot \vec{v}_1 + \frac{18}{5} \vec{S}_1 \cdot \vec{v}_1 \vec{S}_2 \cdot \vec{v}_2 + \\
& \left. 18 \hat{n} \cdot \vec{S}_1 \hat{n} \cdot \vec{S}_2 \vec{v}_1 \cdot \vec{v}_1 - \frac{18}{5} \vec{S}_1 \cdot \vec{S}_2 \vec{v}_1 \cdot \vec{v}_1 - 18 \hat{n} \cdot \vec{S}_1 \hat{n} \cdot \vec{S}_2 \vec{v}_1 \cdot \vec{v}_2 + \frac{18}{5} \vec{S}_1 \cdot \vec{S}_2 \vec{v}_1 \cdot \vec{v}_2 \right) \log \left( \frac{r}{R_\theta} \right) + \\
& \frac{1}{\epsilon_d} \left( \frac{-6 \hat{n} \cdot \vec{S}_2 \hat{n} \cdot \vec{S}_1 \hat{n} \cdot \vec{v}_1 + \frac{6}{5} \vec{S}_1 \cdot \vec{S}_2 \hat{n} \cdot \vec{v}_1 + \frac{6}{5} \hat{n} \cdot \vec{S}_1 \vec{S}_2 \cdot \vec{v}_1 + \frac{6}{5} \hat{n} \cdot \vec{S}_2 \vec{S}_1 \cdot \vec{v}_1}{r^4} + \frac{1}{r^5} \right. \\
& \left( 42 \hat{n} \cdot \vec{S}_1 \hat{n} \cdot \vec{S}_2 (\hat{n} \cdot \vec{v}_1)^2 - 6 \vec{S}_1 \cdot \vec{S}_2 (\hat{n} \cdot \vec{v}_1)^2 - 42 \hat{n} \cdot \vec{S}_1 \hat{n} \cdot \vec{S}_2 \hat{n} \cdot \vec{v}_2 \hat{n} \cdot \vec{v}_1 + 6 \hat{n} \cdot \vec{v}_2 \vec{S}_1 \cdot \vec{S}_2 \hat{n} \cdot \vec{v}_1 - \right. \\
& 12 \hat{n} \cdot \vec{S}_2 \vec{S}_1 \cdot \vec{v}_1 \hat{n} \cdot \vec{v}_1 + 6 \hat{n} \cdot \vec{S}_2 \vec{S}_1 \cdot \vec{v}_2 \hat{n} \cdot \vec{v}_1 - 12 \hat{n} \cdot \vec{S}_1 \vec{S}_2 \cdot \vec{v}_1 \hat{n} \cdot \vec{v}_1 + 6 \hat{n} \cdot \vec{S}_1 \vec{S}_2 \cdot \vec{v}_2 \hat{n} \cdot \vec{v}_1 + \\
& 6 \hat{n} \cdot \vec{S}_2 \hat{n} \cdot \vec{v}_2 \vec{S}_1 \cdot \vec{v}_1 + 6 \hat{n} \cdot \vec{S}_1 \hat{n} \cdot \vec{v}_2 \vec{S}_2 \cdot \vec{v}_1 + \frac{12}{5} \vec{S}_1 \cdot \vec{v}_1 \vec{S}_2 \cdot \vec{v}_1 - \frac{6}{5} \vec{S}_1 \cdot \vec{v}_2 \vec{S}_2 \cdot \vec{v}_1 - \frac{6}{5} \vec{S}_1 \cdot \vec{v}_1 \vec{S}_2 \cdot \vec{v}_2 - \\
& \left. \left. 6 \hat{n} \cdot \vec{S}_1 \hat{n} \cdot \vec{S}_2 \vec{v}_1 \cdot \vec{v}_1 + \frac{6}{5} \vec{S}_1 \cdot \vec{S}_2 \vec{v}_1 \cdot \vec{v}_1 + 6 \hat{n} \cdot \vec{S}_1 \hat{n} \cdot \vec{S}_2 \vec{v}_1 \cdot \vec{v}_2 - \frac{6}{5} \vec{S}_1 \cdot \vec{S}_2 \vec{v}_1 \cdot \vec{v}_2 \right) \right) \Bigg\}
\end{aligned}$$

{DiagS1S2 [3, 1, 24],

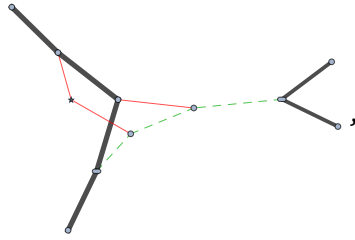

$$\begin{aligned}
& G^3 m_1^2 \left( \frac{1}{r^4} \left( 4 \hat{n} \cdot \vec{S}_2 \hat{n} \cdot \vec{S}_1 \hat{n} \cdot \vec{v}_1 + 4 \hat{n} \cdot \vec{S}_1 \hat{n} \cdot \vec{S}_2 \hat{n} \cdot \vec{v}_1 - \frac{78}{25} \vec{S}_1 \cdot \vec{S}_2 \hat{n} \cdot \vec{v}_1 - \right. \right. \\
& \left. \frac{78}{25} \vec{S}_1 \cdot \vec{S}_2 \hat{n} \cdot \vec{v}_1 - \frac{38}{25} \hat{n} \cdot \vec{S}_2 \vec{S}_1 \cdot \vec{v}_1 + \frac{92}{25} \hat{n} \cdot \vec{S}_1 \vec{S}_2 \cdot \vec{v}_1 - \frac{38}{25} \hat{n} \cdot \vec{S}_2 \vec{S}_1 \cdot \vec{v}_1 + \frac{92}{25} \hat{n} \cdot \vec{S}_1 \vec{S}_2 \cdot \vec{v}_1 \right) + \frac{1}{r^5} \\
& \left( -10 \hat{n} \cdot \vec{S}_1 \hat{n} \cdot \vec{S}_2 (\hat{n} \cdot \vec{v}_1)^2 + \frac{130}{49} \vec{S}_1 \cdot \vec{S}_2 (\hat{n} \cdot \vec{v}_1)^2 + 10 \hat{n} \cdot \vec{S}_1 \hat{n} \cdot \vec{S}_2 \hat{n} \cdot \vec{v}_2 \hat{n} \cdot \vec{v}_1 - 12 \hat{n} \cdot \vec{v}_2 \vec{S}_1 \cdot \vec{S}_2 \hat{n} \cdot \vec{v}_1 + \right. \\
& \frac{344}{49} \hat{n} \cdot \vec{S}_2 \vec{S}_1 \cdot \vec{v}_1 \hat{n} \cdot \vec{v}_1 - 4 \hat{n} \cdot \vec{S}_2 \vec{S}_1 \cdot \vec{v}_2 \hat{n} \cdot \vec{v}_1 - \frac{328}{49} \hat{n} \cdot \vec{S}_1 \vec{S}_2 \cdot \vec{v}_1 \hat{n} \cdot \vec{v}_1 - 4 \hat{n} \cdot \vec{S}_1 \vec{S}_2 \cdot \vec{v}_2 \hat{n} \cdot \vec{v}_1 - \\
& \frac{38}{7} \hat{n} \cdot \vec{S}_1 \cdot \vec{v}_1 \hat{n} \cdot \vec{S}_2 \cdot \vec{v}_1 - 4 \hat{n} \cdot \vec{S}_2 \hat{n} \cdot \vec{v}_2 \vec{S}_1 \cdot \vec{v}_1 + 22 \hat{n} \cdot \vec{S}_1 \hat{n} \cdot \vec{v}_2 \vec{S}_2 \cdot \vec{v}_1 - \frac{1118 \vec{S}_1 \cdot \vec{v}_1 \vec{S}_2 \cdot \vec{v}_1}{1225} - \frac{92}{25} \vec{S}_1 \cdot \vec{v}_2 \vec{S}_2 \cdot \vec{v}_1 + \\
& \left. \frac{38}{25} \vec{S}_1 \cdot \vec{v}_1 \vec{S}_2 \cdot \vec{v}_2 - \frac{276}{49} \hat{n} \cdot \vec{S}_1 \hat{n} \cdot \vec{S}_2 \vec{v}_1 \cdot \vec{v}_1 + \frac{6686 \vec{S}_1 \cdot \vec{S}_2 \vec{v}_1 \cdot \vec{v}_1}{1225} - 4 \hat{n} \cdot \vec{S}_1 \hat{n} \cdot \vec{S}_2 \vec{v}_1 \cdot \vec{v}_2 + \frac{78}{25} \vec{S}_1 \cdot \vec{S}_2 \vec{v}_1 \cdot \vec{v}_2 \right) + \\
& \left( \frac{1}{r^4} \left( 18 \hat{n} \cdot \vec{S}_2 \hat{n} \cdot \vec{S}_1 \hat{n} \cdot \vec{v}_1 + 18 \hat{n} \cdot \vec{S}_1 \hat{n} \cdot \vec{S}_2 \hat{n} \cdot \vec{v}_1 - \frac{18}{5} \vec{S}_1 \cdot \vec{S}_2 \hat{n} \cdot \vec{v}_1 - \frac{18}{5} \vec{S}_1 \cdot \vec{S}_2 \hat{n} \cdot \vec{v}_1 - \right. \right. \\
& \left. \frac{18}{5} \hat{n} \cdot \vec{S}_2 \vec{S}_1 \cdot \vec{v}_1 - \frac{18}{5} \hat{n} \cdot \vec{S}_1 \vec{S}_2 \cdot \vec{v}_1 - \frac{18}{5} \hat{n} \cdot \vec{S}_2 \vec{S}_1 \cdot \vec{v}_1 - \frac{18}{5} \hat{n} \cdot \vec{S}_1 \vec{S}_2 \cdot \vec{v}_1 \right) + \frac{1}{r^5} \\
& \left( -102 \hat{n} \cdot \vec{S}_1 \hat{n} \cdot \vec{S}_2 (\hat{n} \cdot \vec{v}_1)^2 + \frac{102}{7} \vec{S}_1 \cdot \vec{S}_2 (\hat{n} \cdot \vec{v}_1)^2 + 126 \hat{n} \cdot \vec{S}_1 \hat{n} \cdot \vec{S}_2 \hat{n} \cdot \vec{v}_2 \hat{n} \cdot \vec{v}_1 - 18 \hat{n} \cdot \vec{v}_2 \vec{S}_1 \cdot \vec{S}_2 \hat{n} \cdot \vec{v}_1 + \right. \\
& \left. \frac{204}{7} \hat{n} \cdot \vec{S}_2 \vec{S}_1 \cdot \vec{v}_1 \hat{n} \cdot \vec{v}_1 - 18 \hat{n} \cdot \vec{S}_2 \vec{S}_1 \cdot \vec{v}_2 \hat{n} \cdot \vec{v}_1 + \frac{204}{7} \hat{n} \cdot \vec{S}_1 \vec{S}_2 \cdot \vec{v}_1 \hat{n} \cdot \vec{v}_1 - 18 \hat{n} \cdot \vec{S}_1 \vec{S}_2 \cdot \vec{v}_2 \hat{n} \cdot \vec{v}_1 - \right.
\end{aligned}$$

$\{\text{DiagS1S2}[3, 1, 25],$

$$G^3 m_1^2 \left( \frac{1}{r^4} \left( 11 \hat{n} \cdot \vec{S_2} \hat{n} \cdot \vec{S_1} \hat{n} \cdot \vec{v_1} + 11 \hat{n} \cdot \vec{S_1} \hat{n} \cdot \vec{S_2} \hat{n} \cdot \vec{v_1} - \frac{119}{25} \vec{S_1} \cdot \vec{S_2} \hat{n} \cdot \vec{v_1} - \right. \right. \\ \left. \frac{119}{25} \vec{S_1} \cdot \vec{S_2} \hat{n} \cdot \vec{v_1} - \frac{49}{25} \hat{n} \cdot \vec{S_2} \vec{S_1} \cdot \vec{v_1} - \frac{9}{25} \hat{n} \cdot \vec{S_1} \vec{S_2} \cdot \vec{v_1} - \frac{49}{25} \hat{n} \cdot \vec{S_2} \vec{S_1} \cdot \vec{v_1} - \frac{9}{25} \hat{n} \cdot \vec{S_1} \vec{S_2} \cdot \vec{v_1} \right) + \frac{1}{r^5} \\ \left( -68 \hat{n} \cdot \vec{S_1} \hat{n} \cdot \vec{S_2} (\hat{n} \cdot \vec{v_1})^2 + \frac{916}{49} \vec{S_1} \cdot \vec{S_2} (\hat{n} \cdot \vec{v_1})^2 + 83 \hat{n} \cdot \vec{S_1} \hat{n} \cdot \vec{S_2} \hat{n} \cdot \vec{v_2} \hat{n} \cdot \vec{v_1} - 25 \hat{n} \cdot \vec{v_2} \vec{S_1} \cdot \vec{S_2} \hat{n} \cdot \vec{v_1} + \right. \\ \frac{880}{49} \hat{n} \cdot \vec{S_2} \vec{S_1} \cdot \vec{v_1} \hat{n} \cdot \vec{v_1} - 11 \hat{n} \cdot \vec{S_2} \vec{S_1} \cdot \vec{v_2} \hat{n} \cdot \vec{v_1} + \frac{656}{49} \hat{n} \cdot \vec{S_1} \vec{S_2} \cdot \vec{v_1} \hat{n} \cdot \vec{v_1} - 11 \hat{n} \cdot \vec{S_1} \vec{S_2} \cdot \vec{v_2} \hat{n} \cdot \vec{v_1} - \\ \frac{8}{7} \hat{n} \times \vec{S_1} \cdot \vec{v_1} \hat{n} \times \vec{S_2} \cdot \vec{v_1} - 11 \hat{n} \cdot \vec{S_2} \hat{n} \cdot \vec{v_2} \vec{S_1} \cdot \vec{v_1} - 3 \hat{n} \cdot \vec{S_1} \hat{n} \cdot \vec{v_2} \vec{S_2} \cdot \vec{v_1} - \frac{3056 \vec{S_1} \cdot \vec{v_1} \vec{S_2} \cdot \vec{v_1}}{1225} + \frac{9}{25} \vec{S_1} \cdot \vec{v_2} \vec{S_2} \cdot \vec{v_1} + \\ \left. \frac{49}{25} \vec{S_1} \cdot \vec{v_1} \vec{S_2} \cdot \vec{v_2} + \frac{160}{49} \hat{n} \cdot \vec{S_1} \hat{n} \cdot \vec{S_2} \vec{v_1} \cdot \vec{v_1} + \frac{152 \vec{S_1} \cdot \vec{S_2} \vec{v_1} \cdot \vec{v_1}}{1225} - 11 \hat{n} \cdot \vec{S_1} \hat{n} \cdot \vec{S_2} \vec{v_1} \cdot \vec{v_2} + \frac{119}{25} \vec{S_1} \cdot \vec{S_2} \vec{v_1} \cdot \vec{v_2} \right) + \\ \left( \frac{1}{r^4} \left( -6 \hat{n} \cdot \vec{S_2} \hat{n} \cdot \vec{S_1} \hat{n} \cdot \vec{v_1} - 6 \hat{n} \cdot \vec{S_1} \hat{n} \cdot \vec{S_2} \hat{n} \cdot \vec{v_1} + \frac{6}{5} \vec{S_1} \cdot \vec{S_2} \hat{n} \cdot \vec{v_1} + \frac{6}{5} \vec{S_1} \cdot \vec{S_2} \hat{n} \cdot \vec{v_1} + \right. \right. \\ \left. \frac{6}{5} \hat{n} \cdot \vec{S_2} \vec{S_1} \cdot \vec{v_1} + \frac{6}{5} \hat{n} \cdot \vec{S_1} \vec{S_2} \cdot \vec{v_1} + \frac{6}{5} \hat{n} \cdot \vec{S_2} \vec{S_1} \cdot \vec{v_1} + \frac{6}{5} \hat{n} \cdot \vec{S_1} \vec{S_2} \cdot \vec{v_1} \right) + \frac{1}{r^5} \\ \left( 36 \hat{n} \cdot \vec{S_1} \hat{n} \cdot \vec{S_2} (\hat{n} \cdot \vec{v_1})^2 - \frac{36}{7} \vec{S_1} \cdot \vec{S_2} (\hat{n} \cdot \vec{v_1})^2 - 42 \hat{n} \cdot \vec{S_1} \hat{n} \cdot \vec{S_2} \hat{n} \cdot \vec{v_2} \hat{n} \cdot \vec{v_1} + 6 \hat{n} \cdot \vec{v_2} \vec{S_1} \cdot \vec{S_2} \hat{n} \cdot \vec{v_1} - \right. \\ \frac{72}{7} \hat{n} \cdot \vec{S_2} \vec{S_1} \cdot \vec{v_1} \hat{n} \cdot \vec{v_1} + 6 \hat{n} \cdot \vec{S_2} \vec{S_1} \cdot \vec{v_2} \hat{n} \cdot \vec{v_1} - \frac{72}{7} \hat{n} \cdot \vec{S_1} \vec{S_2} \cdot \vec{v_1} \hat{n} \cdot \vec{v_1} + 6 \hat{n} \cdot \vec{S_1} \vec{S_2} \cdot \vec{v_2} \hat{n} \cdot \vec{v_1} + \\ 6 \hat{n} \cdot \vec{S_2} \hat{n} \cdot \vec{v_2} \vec{S_1} \cdot \vec{v_1} + 6 \hat{n} \cdot \vec{S_1} \hat{n} \cdot \vec{v_2} \vec{S_2} \cdot \vec{v_1} + \frac{72}{35} \vec{S_1} \cdot \vec{v_1} \vec{S_2} \cdot \vec{v_1} - \frac{6}{5} \vec{S_1} \cdot \vec{v_2} \vec{S_2} \cdot \vec{v_1} - \frac{6}{5} \vec{S_1} \cdot \vec{v_1} \vec{S_2} \cdot \vec{v_2} - \\ \left. \frac{36}{7} \hat{n} \cdot \vec{S_1} \hat{n} \cdot \vec{S_2} \vec{v_1} \cdot \vec{v_1} + \frac{36}{35} \vec{S_1} \cdot \vec{S_2} \vec{v_1} \cdot \vec{v_1} + 6 \hat{n} \cdot \vec{S_1} \hat{n} \cdot \vec{S_2} \vec{v_1} \cdot \vec{v_2} - \frac{6}{5} \vec{S_1} \cdot \vec{S_2} \vec{v_1} \cdot \vec{v_2} \right) \log \left( \frac{r}{R_\theta} \right) + \\ \frac{1}{\epsilon_d} \left( \frac{1}{r^4} \left( 2 \hat{n} \cdot \vec{S_2} \hat{n} \cdot \vec{S_1} \hat{n} \cdot \vec{v_1} + 2 \hat{n} \cdot \vec{S_1} \hat{n} \cdot \vec{S_2} \hat{n} \cdot \vec{v_1} - \frac{2}{5} \vec{S_1} \cdot \vec{S_2} \hat{n} \cdot \vec{v_1} - \frac{2}{5} \vec{S_1} \cdot \vec{S_2} \hat{n} \cdot \vec{v_1} - \right. \right.$$



$$\left( \frac{2}{5} \hat{n} \cdot \vec{S}_2 \vec{S}_1 \cdot \vec{v}_1 - \frac{2}{5} \hat{n} \cdot \vec{S}_1 \vec{S}_2 \cdot \vec{v}_1 - \frac{2}{5} \hat{n} \cdot \vec{S}_2 \vec{S}_1 \cdot \vec{v}_1 - \frac{2}{5} \hat{n} \cdot \vec{S}_1 \vec{S}_2 \cdot \vec{v}_1 \right) + \frac{1}{r^5} \left( -12 \hat{n} \cdot \vec{S}_1 \hat{n} \cdot \vec{S}_2 (\hat{n} \cdot \vec{v}_1)^2 + \frac{12}{7} \vec{S}_1 \cdot \vec{S}_2 (\hat{n} \cdot \vec{v}_1)^2 + 14 \hat{n} \cdot \vec{S}_1 \hat{n} \cdot \vec{S}_2 \hat{n} \cdot \vec{v}_2 \hat{n} \cdot \vec{v}_1 - 2 \hat{n} \cdot \vec{v}_2 \vec{S}_1 \cdot \vec{S}_2 \hat{n} \cdot \vec{v}_1 + \frac{24}{7} \hat{n} \cdot \vec{S}_2 \vec{S}_1 \cdot \vec{v}_1 \hat{n} \cdot \vec{v}_1 - 2 \hat{n} \cdot \vec{S}_2 \vec{S}_1 \cdot \vec{v}_2 \hat{n} \cdot \vec{v}_1 + \frac{24}{7} \hat{n} \cdot \vec{S}_1 \vec{S}_2 \cdot \vec{v}_1 \hat{n} \cdot \vec{v}_1 - 2 \hat{n} \cdot \vec{S}_1 \vec{S}_2 \cdot \vec{v}_2 \hat{n} \cdot \vec{v}_1 - 2 \hat{n} \cdot \vec{S}_2 \hat{n} \cdot \vec{v}_2 \vec{S}_1 \cdot \vec{v}_1 - 2 \hat{n} \cdot \vec{S}_1 \hat{n} \cdot \vec{v}_2 \vec{S}_2 \cdot \vec{v}_1 - \frac{24}{35} \vec{S}_1 \cdot \vec{v}_1 \vec{S}_2 \cdot \vec{v}_1 + \frac{2}{5} \vec{S}_1 \cdot \vec{v}_2 \vec{S}_2 \cdot \vec{v}_1 + \frac{2}{5} \vec{S}_1 \cdot \vec{v}_1 \vec{S}_2 \cdot \vec{v}_2 + \frac{12}{7} \hat{n} \cdot \vec{S}_1 \hat{n} \cdot \vec{S}_2 \vec{v}_1 \cdot \vec{v}_1 - \frac{12}{35} \vec{S}_1 \cdot \vec{S}_2 \vec{v}_1 \cdot \vec{v}_1 - 2 \hat{n} \cdot \vec{S}_1 \hat{n} \cdot \vec{S}_2 \vec{v}_1 \cdot \vec{v}_2 + \frac{2}{5} \vec{S}_1 \cdot \vec{S}_2 \vec{v}_1 \cdot \vec{v}_2 \right) \right) \Bigg\}$$

{DiagS1S2[3, 1, 26],

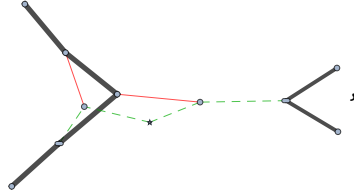

$$G^3 m_1^2 \left( \frac{\hat{n} \cdot \vec{S}_1 \hat{n} \cdot \vec{S}_2 - \frac{5}{3} \vec{S}_1 \cdot \vec{S}_2}{r^3} + \frac{1}{r^4} \left( -5 \hat{n} \cdot \vec{S}_2 \hat{n} \cdot \vec{S}_1 \hat{n} \cdot \vec{v}_1 - 6 \hat{n} \cdot \vec{S}_1 \hat{n} \cdot \vec{S}_2 \hat{n} \cdot \vec{v}_1 + \frac{58}{25} \vec{S}_1 \cdot \vec{S}_2 \hat{n} \cdot \vec{v}_1 + \frac{117}{25} \vec{S}_1 \cdot \vec{S}_2 \hat{n} \cdot \vec{v}_1 + 11 \hat{n} \cdot \vec{S}_1 \hat{n} \cdot \vec{S}_2 \hat{n} \cdot \vec{v}_2 - 7 \hat{n} \cdot \vec{v}_2 \vec{S}_1 \cdot \vec{S}_2 + \frac{18}{25} \hat{n} \cdot \vec{S}_2 \vec{S}_1 \cdot \vec{v}_1 - \hat{n} \cdot \vec{S}_2 \vec{S}_1 \cdot \vec{v}_2 - \frac{13}{25} \hat{n} \cdot \vec{S}_1 \vec{S}_2 \cdot \vec{v}_1 + \frac{7}{25} \hat{n} \cdot \vec{S}_2 \vec{S}_1 \cdot \vec{v}_1 + \frac{38}{25} \hat{n} \cdot \vec{S}_1 \vec{S}_2 \cdot \vec{v}_1 - \hat{n} \cdot \vec{S}_1 \vec{S}_2 \cdot \vec{v}_2 \right) + \frac{1}{r^5} \left( 21 \hat{n} \cdot \vec{S}_1 \hat{n} \cdot \vec{S}_2 (\hat{n} \cdot \vec{v}_1)^2 - \frac{383}{49} \vec{S}_1 \cdot \vec{S}_2 (\hat{n} \cdot \vec{v}_1)^2 - 53 \hat{n} \cdot \vec{S}_1 \hat{n} \cdot \vec{S}_2 \hat{n} \cdot \vec{v}_2 \hat{n} \cdot \vec{v}_1 + 27 \hat{n} \cdot \vec{v}_2 \vec{S}_1 \cdot \vec{S}_2 \hat{n} \cdot \vec{v}_1 - \frac{234}{49} \hat{n} \cdot \vec{S}_2 \vec{S}_1 \cdot \vec{v}_1 \hat{n} \cdot \vec{v}_1 + 5 \hat{n} \cdot \vec{S}_2 \vec{S}_1 \cdot \vec{v}_2 \hat{n} \cdot \vec{v}_1 - \frac{178}{49} \hat{n} \cdot \vec{S}_1 \vec{S}_2 \cdot \vec{v}_1 \hat{n} \cdot \vec{v}_1 + 5 \hat{n} \cdot \vec{S}_1 \vec{S}_2 \cdot \vec{v}_2 \hat{n} \cdot \vec{v}_1 - \frac{12}{7} \hat{n} \cdot \vec{S}_1 \cdot \vec{v}_1 \hat{n} \cdot \vec{S}_2 \cdot \vec{v}_1 + 5 \hat{n} \cdot \vec{S}_2 \hat{n} \cdot \vec{v}_2 \vec{S}_1 \cdot \vec{v}_1 + \hat{n} \cdot \vec{S}_1 \hat{n} \cdot \vec{v}_2 \vec{S}_2 \cdot \vec{v}_1 + \frac{2}{49} \vec{S}_1 \cdot \vec{v}_1 \vec{S}_2 \cdot \vec{v}_1 + \frac{13}{25} \vec{S}_1 \cdot \vec{v}_2 \vec{S}_2 \cdot \vec{v}_1 - \frac{7}{25} \vec{S}_1 \cdot \vec{v}_1 \vec{S}_2 \cdot \vec{v}_2 - \frac{145}{49} \hat{n} \cdot \vec{S}_1 \hat{n} \cdot \vec{S}_2 \vec{v}_1 \cdot \vec{v}_1 + \frac{509}{245} \vec{S}_1 \cdot \vec{S}_2 \vec{v}_1 \cdot \vec{v}_1 + 5 \hat{n} \cdot \vec{S}_1 \hat{n} \cdot \vec{S}_2 \vec{v}_1 \cdot \vec{v}_2 - \frac{117}{25} \vec{S}_1 \cdot \vec{S}_2 \vec{v}_1 \cdot \vec{v}_2 \right) + \left( \frac{2 \vec{S}_1 \cdot \vec{S}_2 - 6 \hat{n} \cdot \vec{S}_1 \hat{n} \cdot \vec{S}_2}{r^3} + \frac{1}{r^4} \left( 18 \hat{n} \cdot \vec{S}_2 \hat{n} \cdot \vec{S}_1 \hat{n} \cdot \vec{v}_1 + 12 \hat{n} \cdot \vec{S}_1 \hat{n} \cdot \vec{S}_2 \hat{n} \cdot \vec{v}_1 - \frac{12}{5} \vec{S}_1 \cdot \vec{S}_2 \hat{n} \cdot \vec{v}_1 - \frac{18}{5} \vec{S}_1 \cdot \vec{S}_2 \hat{n} \cdot \vec{v}_1 - 30 \hat{n} \cdot \vec{S}_1 \hat{n} \cdot \vec{S}_2 \hat{n} \cdot \vec{v}_2 + 6 \hat{n} \cdot \vec{v}_2 \vec{S}_1 \cdot \vec{S}_2 - \frac{12}{5} \hat{n} \cdot \vec{S}_2 \vec{S}_1 \cdot \vec{v}_1 + 6 \hat{n} \cdot \vec{S}_2 \vec{S}_1 \cdot \vec{v}_2 - \frac{18}{5} \hat{n} \cdot \vec{S}_1 \vec{S}_2 \cdot \vec{v}_1 - \frac{18}{5} \hat{n} \cdot \vec{S}_2 \vec{S}_1 \cdot \vec{v}_1 - \frac{12}{5} \hat{n} \cdot \vec{S}_1 \vec{S}_2 \cdot \vec{v}_1 + 6 \hat{n} \cdot \vec{S}_1 \vec{S}_2 \cdot \vec{v}_2 \right) + \frac{1}{r^5} \left( -30 \hat{n} \cdot \vec{S}_1 \hat{n} \cdot \vec{S}_2 (\hat{n} \cdot \vec{v}_1)^2 + \frac{30}{7} \vec{S}_1 \cdot \vec{S}_2 (\hat{n} \cdot \vec{v}_1)^2 + 126 \hat{n} \cdot \vec{S}_1 \hat{n} \cdot \vec{S}_2 \hat{n} \cdot \vec{v}_2 \hat{n} \cdot \vec{v}_1 - 18 \hat{n} \cdot \vec{v}_2 \vec{S}_1 \cdot \vec{S}_2 \hat{n} \cdot \vec{v}_1 + \frac{60}{7} \hat{n} \cdot \vec{S}_2 \vec{S}_1 \cdot \vec{v}_1 \hat{n} \cdot \vec{v}_1 - 18 \hat{n} \cdot \vec{S}_2 \vec{S}_1 \cdot \vec{v}_2 \hat{n} \cdot \vec{v}_1 + \frac{60}{7} \hat{n} \cdot \vec{S}_1 \vec{S}_2 \cdot \vec{v}_1 \hat{n} \cdot \vec{v}_1 - 18 \hat{n} \cdot \vec{S}_1 \vec{S}_2 \cdot \vec{v}_2 \hat{n} \cdot \vec{v}_1 - 18 \hat{n} \cdot \vec{S}_2 \hat{n} \cdot \vec{v}_2 \vec{S}_1 \cdot \vec{v}_1 - 18 \hat{n} \cdot \vec{S}_1 \hat{n} \cdot \vec{v}_2 \vec{S}_2 \cdot \vec{v}_1 - \frac{12}{7} \vec{S}_1 \cdot \vec{v}_1 \vec{S}_2 \cdot \vec{v}_1 + \frac{18}{5} \vec{S}_1 \cdot \vec{v}_2 \vec{S}_2 \cdot \vec{v}_1 + \frac{18}{5} \vec{S}_1 \cdot \vec{v}_1 \vec{S}_2 \cdot \vec{v}_2 + \frac{30}{7} \hat{n} \cdot \vec{S}_1 \hat{n} \cdot \vec{S}_2 \vec{v}_1 \cdot \vec{v}_1 - \frac{6}{7} \vec{S}_1 \cdot \vec{S}_2 \vec{v}_1 \cdot \vec{v}_1 - 18 \hat{n} \cdot \vec{S}_1 \hat{n} \cdot \vec{S}_2 \vec{v}_1 \cdot \vec{v}_2 + \frac{18}{5} \vec{S}_1 \cdot \vec{S}_2 \vec{v}_1 \cdot \vec{v}_2 \right) \Bigg) \log \left( \frac{r}{R_0} \right) +$$

$$\begin{aligned}
& \frac{1}{\epsilon_d} \left( \frac{2 \hat{n} \cdot \vec{S}_1 \hat{n} \cdot \vec{S}_2 - \frac{2}{3} \vec{S}_1 \cdot \vec{S}_2}{r^3} + \frac{1}{r^4} \left( -6 \hat{n} \cdot \vec{S}_2 \hat{n} \cdot \vec{S}_1 \hat{n} \cdot \vec{v}_1 - 4 \hat{n} \cdot \vec{S}_1 \hat{n} \cdot \vec{S}_2 \hat{n} \cdot \vec{v}_1 + \frac{4}{5} \vec{S}_1 \cdot \vec{S}_2 \hat{n} \cdot \vec{v}_1 + \right. \right. \\
& \quad \frac{6}{5} \vec{S}_1 \cdot \vec{S}_2 \hat{n} \cdot \vec{v}_1 + 10 \hat{n} \cdot \vec{S}_1 \hat{n} \cdot \vec{S}_2 \hat{n} \cdot \vec{v}_2 - 2 \hat{n} \cdot \vec{v}_2 \vec{S}_1 \cdot \vec{S}_2 + \frac{4}{5} \hat{n} \cdot \vec{S}_2 \vec{S}_1 \cdot \vec{v}_1 - \\
& \quad \left. \left. 2 \hat{n} \cdot \vec{S}_2 \vec{S}_1 \cdot \vec{v}_2 + \frac{6}{5} \hat{n} \cdot \vec{S}_1 \vec{S}_2 \cdot \vec{v}_1 + \frac{6}{5} \hat{n} \cdot \vec{S}_2 \vec{S}_1 \cdot \vec{v}_1 + \frac{4}{5} \hat{n} \cdot \vec{S}_1 \vec{S}_2 \cdot \vec{v}_1 - 2 \hat{n} \cdot \vec{S}_1 \vec{S}_2 \cdot \vec{v}_2 \right) + \frac{1}{r^5} \right. \\
& \quad \left( 10 \hat{n} \cdot \vec{S}_1 \hat{n} \cdot \vec{S}_2 (\hat{n} \cdot \vec{v}_1)^2 - \frac{10}{7} \vec{S}_1 \cdot \vec{S}_2 (\hat{n} \cdot \vec{v}_1)^2 - 42 \hat{n} \cdot \vec{S}_1 \hat{n} \cdot \vec{S}_2 \hat{n} \cdot \vec{v}_2 \hat{n} \cdot \vec{v}_1 + 6 \hat{n} \cdot \vec{v}_2 \vec{S}_1 \cdot \vec{S}_2 \hat{n} \cdot \vec{v}_1 - \right. \\
& \quad \frac{20}{7} \hat{n} \cdot \vec{S}_2 \vec{S}_1 \cdot \vec{v}_1 \hat{n} \cdot \vec{v}_1 + 6 \hat{n} \cdot \vec{S}_2 \vec{S}_1 \cdot \vec{v}_2 \hat{n} \cdot \vec{v}_1 - \frac{20}{7} \hat{n} \cdot \vec{S}_1 \vec{S}_2 \cdot \vec{v}_1 \hat{n} \cdot \vec{v}_1 + 6 \hat{n} \cdot \vec{S}_1 \vec{S}_2 \cdot \vec{v}_2 \hat{n} \cdot \vec{v}_1 + \\
& \quad \left. 6 \hat{n} \cdot \vec{S}_2 \hat{n} \cdot \vec{v}_2 \vec{S}_1 \cdot \vec{v}_1 + 6 \hat{n} \cdot \vec{S}_1 \hat{n} \cdot \vec{v}_2 \vec{S}_2 \cdot \vec{v}_1 + \frac{4}{7} \vec{S}_1 \cdot \vec{v}_1 \vec{S}_2 \cdot \vec{v}_1 - \frac{6}{5} \vec{S}_1 \cdot \vec{v}_2 \vec{S}_2 \cdot \vec{v}_1 - \frac{6}{5} \vec{S}_1 \cdot \vec{v}_1 \vec{S}_2 \cdot \vec{v}_2 - \right. \\
& \quad \left. \left. \frac{10}{7} \hat{n} \cdot \vec{S}_1 \hat{n} \cdot \vec{S}_2 \vec{v}_1 \cdot \vec{v}_1 + \frac{2}{7} \vec{S}_1 \cdot \vec{S}_2 \vec{v}_1 \cdot \vec{v}_1 + 6 \hat{n} \cdot \vec{S}_1 \hat{n} \cdot \vec{S}_2 \vec{v}_1 \cdot \vec{v}_2 - \frac{6}{5} \vec{S}_1 \cdot \vec{S}_2 \vec{v}_1 \cdot \vec{v}_2 \right) \right) \Bigg\}
\end{aligned}$$

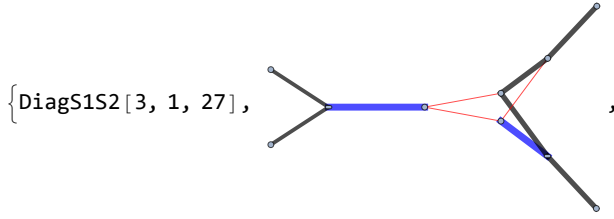

$$\frac{G^3 m_1^2 \left( -\frac{4}{7} \hat{n} \times \vec{S}_1 \cdot \vec{v}_1 \hat{n} \times \vec{S}_2 \cdot \vec{v}_2 + \frac{1}{14} \vec{S}_1 \cdot \vec{S}_2 \hat{n} \cdot \vec{v}_1 \hat{n} \cdot \vec{v}_2 - \frac{1}{14} \hat{n} \cdot \vec{S}_1 \hat{n} \cdot \vec{v}_2 \vec{S}_2 \cdot \vec{v}_1 - \frac{1}{10} \vec{S}_1 \cdot \vec{v}_2 \vec{S}_2 \cdot \vec{v}_1 + \frac{1}{10} \vec{S}_1 \cdot \vec{S}_2 \vec{v}_1 \cdot \vec{v}_2 \right)}{r^5} \Bigg\}$$

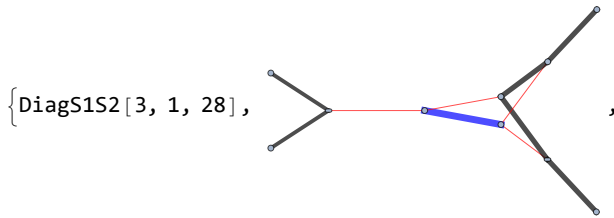

$$\frac{G^3 m_1^2 \left( -8 \hat{n} \times \vec{S}_1 \cdot \vec{v}_1 \hat{n} \times \vec{S}_2 \cdot \vec{v}_2 - \frac{8}{5} \vec{S}_1 \cdot \vec{v}_2 \vec{S}_2 \cdot \vec{v}_1 + \frac{8}{5} \vec{S}_1 \cdot \vec{S}_2 \vec{v}_1 \cdot \vec{v}_2 \right)}{r^5} \Bigg\}$$

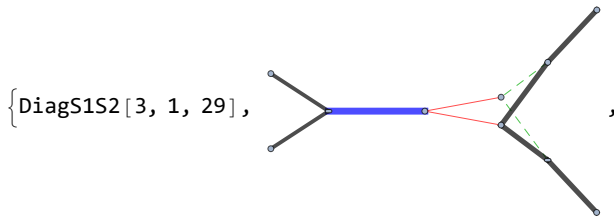

$$\frac{G^3 m_1^2 \left( \frac{16}{7} \hat{n} \times \vec{S}_1 \cdot \vec{v}_1 \hat{n} \times \vec{S}_2 \cdot \vec{v}_2 - \frac{2}{7} \vec{S}_1 \cdot \vec{S}_2 \hat{n} \cdot \vec{v}_1 \hat{n} \cdot \vec{v}_2 + \frac{2}{7} \hat{n} \cdot \vec{S}_1 \hat{n} \cdot \vec{v}_2 \vec{S}_2 \cdot \vec{v}_1 + \frac{2}{5} \vec{S}_1 \cdot \vec{v}_2 \vec{S}_2 \cdot \vec{v}_1 - \frac{2}{5} \vec{S}_1 \cdot \vec{S}_2 \vec{v}_1 \cdot \vec{v}_2 \right)}{r^5} \Bigg\}$$

{DiagS1S2 [3, 1, 30],

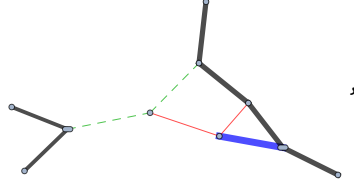

$$\frac{G^3 m_1^2 \left( -6 \hat{n} \times \vec{S}_1 \cdot \vec{v}_1 \hat{n} \times \vec{S}_2 \cdot \vec{v}_1 - 2 \vec{S}_1 \cdot \vec{S}_2 (\hat{n} \cdot \vec{v}_1)^2 + 2 \hat{n} \cdot \vec{S}_1 \hat{n} \cdot \vec{v}_1 \vec{S}_2 \cdot \vec{v}_1 - \frac{8}{5} \vec{S}_1 \cdot \vec{v}_1 \vec{S}_2 \cdot \vec{v}_1 + \frac{8}{5} \vec{S}_1 \cdot \vec{S}_2 \vec{v}_1 \cdot \vec{v}_1 \right)}{r^5}$$

{DiagS1S2 [3, 1, 31],

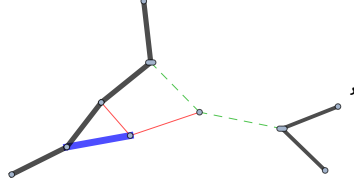

$$\begin{aligned} G^3 m_1^2 \left( \frac{1}{r^5 \in_d} \left( -16 \hat{n} \cdot \vec{S}_1 \hat{n} \cdot \vec{S}_2 (\hat{n} \cdot \vec{v}_1)^2 + \frac{16}{7} \vec{S}_1 \cdot \vec{S}_2 (\hat{n} \cdot \vec{v}_1)^2 + \frac{32}{7} \hat{n} \cdot \vec{S}_2 \hat{n} \cdot \vec{v}_1 \vec{S}_1 \cdot \vec{v}_1 + \right. \right. \\ \left. \frac{32}{7} \hat{n} \cdot \vec{S}_1 \hat{n} \cdot \vec{v}_1 \vec{S}_2 \cdot \vec{v}_1 + \frac{16}{7} \vec{v}_1 \cdot \vec{v}_1 \hat{n} \cdot \vec{S}_1 \hat{n} \cdot \vec{S}_2 - \frac{32}{35} \vec{S}_1 \cdot \vec{v}_1 \vec{S}_2 \cdot \vec{v}_1 - \frac{16}{35} \vec{S}_1 \cdot \vec{S}_2 \vec{v}_1 \cdot \vec{v}_1 \right) + \\ \left. \frac{1}{r^5} \log \left( \frac{r}{R_0} \right) \left( 48 \hat{n} \cdot \vec{S}_1 \hat{n} \cdot \vec{S}_2 (\hat{n} \cdot \vec{v}_1)^2 - \frac{48}{7} \vec{S}_1 \cdot \vec{S}_2 (\hat{n} \cdot \vec{v}_1)^2 - \frac{96}{7} \hat{n} \cdot \vec{S}_2 \hat{n} \cdot \vec{v}_1 \vec{S}_1 \cdot \vec{v}_1 - \right. \right. \\ \left. \frac{96}{7} \hat{n} \cdot \vec{S}_1 \hat{n} \cdot \vec{v}_1 \vec{S}_2 \cdot \vec{v}_1 - \frac{48}{7} \vec{v}_1 \cdot \vec{v}_1 \hat{n} \cdot \vec{S}_1 \hat{n} \cdot \vec{S}_2 + \frac{96}{35} \vec{S}_1 \cdot \vec{v}_1 \vec{S}_2 \cdot \vec{v}_1 + \frac{48}{35} \vec{S}_1 \cdot \vec{S}_2 \vec{v}_1 \cdot \vec{v}_1 \right) + \frac{1}{r^5} \\ \left. \left( -\frac{48}{7} \hat{n} \times \vec{S}_1 \cdot \vec{v}_1 \hat{n} \times \vec{S}_2 \cdot \vec{v}_1 - 16 \hat{n} \cdot \vec{S}_1 \hat{n} \cdot \vec{S}_2 (\hat{n} \cdot \vec{v}_1)^2 - \frac{608}{49} \vec{S}_1 \cdot \vec{S}_2 (\hat{n} \cdot \vec{v}_1)^2 + \frac{128}{49} \hat{n} \cdot \vec{S}_2 \hat{n} \cdot \vec{v}_1 \vec{S}_1 \cdot \vec{v}_1 + \right. \right. \\ \left. \left. \frac{1136}{49} \hat{n} \cdot \vec{S}_1 \hat{n} \cdot \vec{v}_1 \vec{S}_2 \cdot \vec{v}_1 - \frac{440}{49} \vec{v}_1 \cdot \vec{v}_1 \hat{n} \cdot \vec{S}_1 \hat{n} \cdot \vec{S}_2 - \frac{6688 \vec{S}_1 \cdot \vec{v}_1 \vec{S}_2 \cdot \vec{v}_1}{1225} + \frac{12616 \vec{S}_1 \cdot \vec{S}_2 \vec{v}_1 \cdot \vec{v}_1}{1225} \right) \right) \Bigg\} \end{aligned}$$

{DiagS1S2 [3, 1, 32],

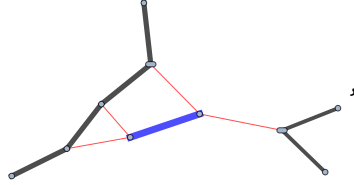

$$\frac{G^3 m_1^2 \left( -12 \hat{n} \times \vec{S}_1 \cdot \vec{v}_1 \hat{n} \times \vec{S}_2 \cdot \vec{v}_2 - \frac{12}{5} \vec{S}_1 \cdot \vec{v}_2 \vec{S}_2 \cdot \vec{v}_1 + \frac{12}{5} \vec{S}_1 \cdot \vec{S}_2 \vec{v}_1 \cdot \vec{v}_2 \right)}{r^5}$$

{DiagS1S2 [3, 1, 33],

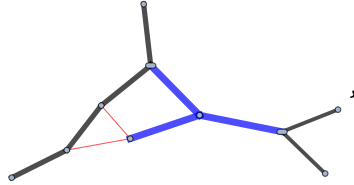

$$\begin{aligned} G^3 m_1^2 \left( \frac{1}{r^5 \in_d} \left( -3 \hat{n} \cdot \vec{S}_1 \hat{n} \cdot \vec{S}_2 \hat{n} \cdot \vec{v}_1 \hat{n} \cdot \vec{v}_2 + \frac{3}{7} \hat{n} \cdot \vec{v}_1 \vec{S}_1 \cdot \vec{S}_2 \hat{n} \cdot \vec{v}_2 + \right. \right. \\ \left. \frac{3}{7} \hat{n} \cdot \vec{S}_2 \vec{S}_1 \cdot \vec{v}_1 \hat{n} \cdot \vec{v}_2 + \frac{3}{7} \hat{n} \cdot \vec{S}_1 \vec{S}_2 \cdot \vec{v}_1 \hat{n} \cdot \vec{v}_2 + \frac{3}{7} \hat{n} \cdot \vec{S}_2 \hat{n} \cdot \vec{v}_1 \vec{S}_1 \cdot \vec{v}_2 - \frac{3}{35} \vec{S}_1 \cdot \vec{v}_2 \vec{S}_2 \cdot \vec{v}_1 + \right. \\ \left. \frac{3}{7} \hat{n} \cdot \vec{S}_1 \hat{n} \cdot \vec{v}_1 \vec{S}_2 \cdot \vec{v}_2 - \frac{3}{35} \vec{S}_1 \cdot \vec{v}_1 \vec{S}_2 \cdot \vec{v}_2 + \frac{3}{7} \hat{n} \cdot \vec{S}_1 \hat{n} \cdot \vec{S}_2 \vec{v}_1 \cdot \vec{v}_2 - \frac{3}{35} \vec{S}_1 \cdot \vec{S}_2 \vec{v}_1 \cdot \vec{v}_2 \right) + \frac{1}{r^5} \end{aligned}$$

$$\begin{aligned}
& \left( \frac{3}{7} \hat{n} \times \vec{S}_1 \cdot \vec{v}_2 \hat{n} \times \vec{S}_2 \cdot \vec{v}_1 - \frac{12}{7} \hat{n} \times \vec{S}_1 \cdot \vec{v}_1 \hat{n} \times \vec{S}_2 \cdot \vec{v}_2 - 9 \hat{n} \cdot \vec{S}_1 \hat{n} \cdot \vec{S}_2 \hat{n} \cdot \vec{v}_1 \hat{n} \cdot \vec{v}_2 + \frac{26}{49} \hat{n} \cdot \vec{v}_1 \hat{n} \cdot \vec{v}_2 \vec{S}_1 \cdot \vec{S}_2 + \right. \\
& \frac{54}{49} \hat{n} \cdot \vec{S}_2 \hat{n} \cdot \vec{v}_2 \vec{S}_1 \cdot \vec{v}_1 + \frac{54}{49} \hat{n} \cdot \vec{S}_2 \hat{n} \cdot \vec{v}_1 \vec{S}_1 \cdot \vec{v}_2 + \frac{145}{49} \hat{n} \cdot \vec{S}_1 \hat{n} \cdot \vec{v}_2 \vec{S}_2 \cdot \vec{v}_1 - \frac{1082 \vec{S}_1 \cdot \vec{v}_2 \vec{S}_2 \cdot \vec{v}_1}{1225} + \\
& \left. \frac{54}{49} \hat{n} \cdot \vec{S}_1 \hat{n} \cdot \vec{v}_1 \vec{S}_2 \cdot \vec{v}_2 - \frac{102 \vec{S}_1 \cdot \vec{v}_1 \vec{S}_2 \cdot \vec{v}_2}{1225} + \frac{33}{49} \hat{n} \cdot \vec{S}_1 \hat{n} \cdot \vec{S}_2 \vec{v}_1 \cdot \vec{v}_2 + \frac{563 \vec{S}_1 \cdot \vec{S}_2 \vec{v}_1 \cdot \vec{v}_2}{1225} \right) + \frac{1}{r^5} \\
& \left( 9 \hat{n} \cdot \vec{S}_1 \hat{n} \cdot \vec{S}_2 \hat{n} \cdot \vec{v}_1 \hat{n} \cdot \vec{v}_2 - \frac{9}{7} \hat{n} \cdot \vec{v}_1 \vec{S}_1 \cdot \vec{S}_2 \hat{n} \cdot \vec{v}_2 - \frac{9}{7} \hat{n} \cdot \vec{S}_2 \vec{S}_1 \cdot \vec{v}_1 \hat{n} \cdot \vec{v}_2 - \frac{9}{7} \hat{n} \cdot \vec{S}_1 \vec{S}_2 \cdot \vec{v}_1 \hat{n} \cdot \vec{v}_2 - \right. \\
& \frac{9}{7} \hat{n} \cdot \vec{S}_2 \hat{n} \cdot \vec{v}_1 \vec{S}_1 \cdot \vec{v}_2 + \frac{9}{35} \vec{S}_1 \cdot \vec{v}_2 \vec{S}_2 \cdot \vec{v}_1 - \frac{9}{7} \hat{n} \cdot \vec{S}_1 \hat{n} \cdot \vec{v}_1 \vec{S}_2 \cdot \vec{v}_2 + \\
& \left. \frac{9}{35} \vec{S}_1 \cdot \vec{v}_1 \vec{S}_2 \cdot \vec{v}_2 - \frac{9}{7} \hat{n} \cdot \vec{S}_1 \hat{n} \cdot \vec{S}_2 \vec{v}_1 \cdot \vec{v}_2 + \frac{9}{35} \vec{S}_1 \cdot \vec{S}_2 \vec{v}_1 \cdot \vec{v}_2 \right) \log \left( \frac{r}{R_\theta} \right) \Bigg\}
\end{aligned}$$

{DiagS1S2 [3, 1, 34],

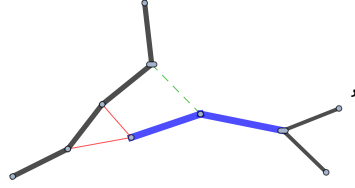

$$\begin{aligned}
& G^3 m_1^2 \left( \frac{1}{r^4} \left( -\frac{3}{4} \hat{n} \cdot \vec{a}_2 \hat{n} \cdot \vec{S}_1 \hat{n} \cdot \vec{S}_2 + \frac{9}{4} \hat{n} \cdot \vec{S}_1 \hat{n} \cdot \vec{v}_2 \hat{n} \cdot \vec{S}_2 - \frac{9}{20} \vec{S}_1 \cdot \vec{v}_2 \hat{n} \cdot \vec{S}_2 + \right. \right. \\
& \frac{3}{100} \vec{S}_1 \cdot \vec{a}_2 \hat{n} \cdot \vec{S}_2 - \frac{3}{4} \hat{n} \cdot \vec{S}_2 \hat{n} \cdot \vec{S}_1 \hat{n} \cdot \vec{v}_2 - \frac{9}{20} \hat{n} \cdot \vec{v}_2 \vec{S}_1 \cdot \vec{S}_2 + \frac{3}{100} \hat{n} \cdot \vec{S}_1 \vec{S}_2 \cdot \vec{v}_2 + \\
& \left. \frac{63}{100} \hat{n} \cdot \vec{v}_2 \vec{S}_1 \cdot \vec{S}_2 + \frac{63}{100} \hat{n} \cdot \vec{a}_2 \vec{S}_1 \cdot \vec{S}_2 + \frac{3}{100} \hat{n} \cdot \vec{S}_2 \vec{S}_1 \cdot \vec{v}_2 + \frac{3}{100} \hat{n} \cdot \vec{S}_1 \vec{S}_2 \cdot \vec{a}_2 - \frac{9}{20} \hat{n} \cdot \vec{S}_1 \vec{S}_2 \cdot \vec{v}_2 \right) + \\
& \frac{1}{r^5} \left( -\frac{33}{4} \hat{n} \cdot \vec{S}_1 \hat{n} \cdot \vec{S}_2 (\hat{n} \cdot \vec{v}_2)^2 + \frac{15}{4} \vec{S}_1 \cdot \vec{S}_2 (\hat{n} \cdot \vec{v}_2)^2 + \frac{117}{4} \hat{n} \cdot \vec{S}_1 \hat{n} \cdot \vec{S}_2 \hat{n} \cdot \vec{v}_1 \hat{n} \cdot \vec{v}_2 - \right. \\
& \frac{1913}{196} \hat{n} \cdot \vec{v}_1 \vec{S}_1 \cdot \vec{S}_2 \hat{n} \cdot \vec{v}_2 - \frac{681}{196} \hat{n} \cdot \vec{S}_2 \vec{S}_1 \cdot \vec{v}_1 \hat{n} \cdot \vec{v}_2 + \frac{3}{2} \hat{n} \cdot \vec{S}_2 \vec{S}_1 \cdot \vec{v}_2 \hat{n} \cdot \vec{v}_2 - \frac{415}{196} \hat{n} \cdot \vec{S}_1 \vec{S}_2 \cdot \vec{v}_1 \hat{n} \cdot \vec{v}_2 + \\
& \frac{3}{2} \hat{n} \cdot \vec{S}_1 \vec{S}_2 \cdot \vec{v}_2 \hat{n} \cdot \vec{v}_2 + \frac{6}{7} \hat{n} \times \vec{S}_1 \cdot \vec{v}_2 \hat{n} \times \vec{S}_2 \cdot \vec{v}_1 - \frac{16}{7} \hat{n} \times \vec{S}_1 \cdot \vec{v}_1 \hat{n} \times \vec{S}_2 \cdot \vec{v}_2 - \frac{681}{196} \hat{n} \cdot \vec{S}_2 \hat{n} \cdot \vec{v}_1 \vec{S}_1 \cdot \vec{v}_2 - \\
& \frac{1131 \vec{S}_1 \cdot \vec{v}_2 \vec{S}_2 \cdot \vec{v}_1}{4900} - \frac{681}{196} \hat{n} \cdot \vec{S}_1 \hat{n} \cdot \vec{v}_1 \vec{S}_2 \cdot \vec{v}_2 + \frac{3279 \vec{S}_1 \cdot \vec{v}_1 \vec{S}_2 \cdot \vec{v}_2}{4900} - \frac{3}{50} \vec{S}_1 \cdot \vec{v}_2 \vec{S}_2 \cdot \vec{v}_2 - \\
& \left. \frac{849}{196} \hat{n} \cdot \vec{S}_1 \hat{n} \cdot \vec{S}_2 \vec{v}_1 \cdot \vec{v}_2 + \frac{12519 \vec{S}_1 \cdot \vec{S}_2 \vec{v}_1 \cdot \vec{v}_2}{4900} + \frac{3}{4} \hat{n} \cdot \vec{S}_1 \hat{n} \cdot \vec{S}_2 \vec{v}_2 \cdot \vec{v}_2 - \frac{63}{100} \vec{S}_1 \cdot \vec{S}_2 \vec{v}_2 \cdot \vec{v}_2 \right) + \\
& \left( \frac{1}{r^4} \left( 3 \hat{n} \cdot \vec{a}_2 \hat{n} \cdot \vec{S}_1 \hat{n} \cdot \vec{S}_2 - \frac{3}{5} \vec{S}_1 \cdot \vec{a}_2 \hat{n} \cdot \vec{S}_2 + 3 \hat{n} \cdot \vec{S}_2 \hat{n} \cdot \vec{S}_1 \hat{n} \cdot \vec{v}_2 - \frac{3}{5} \hat{n} \cdot \vec{S}_1 \vec{S}_2 \cdot \vec{v}_2 - \right. \right. \\
& \left. \frac{3}{5} \hat{n} \cdot \vec{v}_2 \vec{S}_1 \cdot \vec{S}_2 - \frac{3}{5} \hat{n} \cdot \vec{a}_2 \vec{S}_1 \cdot \vec{S}_2 - \frac{3}{5} \hat{n} \cdot \vec{S}_2 \vec{S}_1 \cdot \vec{v}_2 - \frac{3}{5} \hat{n} \cdot \vec{S}_1 \vec{S}_2 \cdot \vec{a}_2 \right) + \frac{1}{r^5} \\
& \left( 21 \hat{n} \cdot \vec{S}_1 \hat{n} \cdot \vec{S}_2 (\hat{n} \cdot \vec{v}_2)^2 - 3 \vec{S}_1 \cdot \vec{S}_2 (\hat{n} \cdot \vec{v}_2)^2 - \frac{69}{2} \hat{n} \cdot \vec{S}_1 \hat{n} \cdot \vec{S}_2 \hat{n} \cdot \vec{v}_1 \hat{n} \cdot \vec{v}_2 + \frac{69}{14} \hat{n} \cdot \vec{v}_1 \vec{S}_1 \cdot \vec{S}_2 \hat{n} \cdot \vec{v}_2 + \right. \\
& \frac{69}{14} \hat{n} \cdot \vec{S}_2 \vec{S}_1 \cdot \vec{v}_1 \hat{n} \cdot \vec{v}_2 - 6 \hat{n} \cdot \vec{S}_2 \vec{S}_1 \cdot \vec{v}_2 \hat{n} \cdot \vec{v}_2 + \frac{69}{14} \hat{n} \cdot \vec{S}_1 \vec{S}_2 \cdot \vec{v}_1 \hat{n} \cdot \vec{v}_2 - 6 \hat{n} \cdot \vec{S}_1 \vec{S}_2 \cdot \vec{v}_2 \hat{n} \cdot \vec{v}_2 + \\
& \frac{69}{14} \hat{n} \cdot \vec{S}_2 \hat{n} \cdot \vec{v}_1 \vec{S}_1 \cdot \vec{v}_2 - \frac{69}{70} \vec{S}_1 \cdot \vec{v}_2 \vec{S}_2 \cdot \vec{v}_1 + \frac{69}{14} \hat{n} \cdot \vec{S}_1 \hat{n} \cdot \vec{v}_1 \vec{S}_2 \cdot \vec{v}_2 - \frac{69}{70} \vec{S}_1 \cdot \vec{v}_1 \vec{S}_2 \cdot \vec{v}_2 + \frac{6}{5} \vec{S}_1 \cdot \vec{v}_2 \vec{S}_2 \cdot \vec{v}_2 + \\
& \left. \frac{69}{14} \hat{n} \cdot \vec{S}_1 \hat{n} \cdot \vec{S}_2 \vec{v}_1 \cdot \vec{v}_2 - \frac{69}{70} \vec{S}_1 \cdot \vec{S}_2 \vec{v}_1 \cdot \vec{v}_2 - 3 \hat{n} \cdot \vec{S}_1 \hat{n} \cdot \vec{S}_2 \vec{v}_2 \cdot \vec{v}_2 + \frac{3}{5} \vec{S}_1 \cdot \vec{S}_2 \vec{v}_2 \cdot \vec{v}_2 \right) \log \left( \frac{r}{R_\theta} \right) + \\
& \frac{1}{r^4} \left( \frac{1}{r^4} \left( -(\hat{n} \cdot \vec{a}_2) \hat{n} \cdot \vec{S}_1 \hat{n} \cdot \vec{S}_2 + \frac{1}{5} \vec{S}_1 \cdot \vec{a}_2 \hat{n} \cdot \vec{S}_2 - \hat{n} \cdot \vec{S}_2 \hat{n} \cdot \vec{S}_1 \hat{n} \cdot \vec{v}_2 + \frac{1}{5} \hat{n} \cdot \vec{S}_1 \vec{S}_2 \cdot \vec{v}_2 + \right. \right.
\end{aligned}$$

$$\left. \begin{aligned} & \frac{1}{5} \hat{n} \cdot \vec{v}_2 \vec{S}_1 \cdot \vec{S}_2 + \frac{1}{5} \hat{n} \cdot \vec{a}_2 \vec{S}_1 \cdot \vec{S}_2 + \frac{1}{5} \hat{n} \cdot \vec{S}_2 \vec{S}_1 \cdot \vec{v}_2 + \frac{1}{5} \hat{n} \cdot \vec{S}_1 \vec{S}_2 \cdot \vec{a}_2 \right) + \frac{1}{r^5} \\ & \left( -7 \hat{n} \cdot \vec{S}_1 \hat{n} \cdot \vec{S}_2 (\hat{n} \cdot \vec{v}_2)^2 + \vec{S}_1 \cdot \vec{S}_2 (\hat{n} \cdot \vec{v}_2)^2 + \frac{23}{2} \hat{n} \cdot \vec{S}_1 \hat{n} \cdot \vec{S}_2 \hat{n} \cdot \vec{v}_1 \hat{n} \cdot \vec{v}_2 - \frac{23}{14} \hat{n} \cdot \vec{v}_1 \vec{S}_1 \cdot \vec{S}_2 \hat{n} \cdot \vec{v}_2 - \right. \\ & \frac{23}{14} \hat{n} \cdot \vec{S}_2 \vec{S}_1 \cdot \vec{v}_1 \hat{n} \cdot \vec{v}_2 + 2 \hat{n} \cdot \vec{S}_2 \vec{S}_1 \cdot \vec{v}_2 \hat{n} \cdot \vec{v}_2 - \frac{23}{14} \hat{n} \cdot \vec{S}_1 \vec{S}_2 \cdot \vec{v}_1 \hat{n} \cdot \vec{v}_2 + 2 \hat{n} \cdot \vec{S}_1 \vec{S}_2 \cdot \vec{v}_2 \hat{n} \cdot \vec{v}_2 - \\ & \frac{23}{14} \hat{n} \cdot \vec{S}_2 \hat{n} \cdot \vec{v}_1 \vec{S}_1 \cdot \vec{v}_2 + \frac{23}{70} \vec{S}_1 \cdot \vec{v}_2 \vec{S}_2 \cdot \vec{v}_1 - \frac{23}{14} \hat{n} \cdot \vec{S}_1 \hat{n} \cdot \vec{v}_1 \vec{S}_2 \cdot \vec{v}_2 + \frac{23}{70} \vec{S}_1 \cdot \vec{v}_1 \vec{S}_2 \cdot \vec{v}_2 - \\ & \left. \frac{2}{5} \vec{S}_1 \cdot \vec{v}_2 \vec{S}_2 \cdot \vec{v}_2 - \frac{23}{14} \hat{n} \cdot \vec{S}_1 \hat{n} \cdot \vec{S}_2 \vec{v}_1 \cdot \vec{v}_2 + \frac{23}{70} \vec{S}_1 \cdot \vec{S}_2 \vec{v}_1 \cdot \vec{v}_2 + \hat{n} \cdot \vec{S}_1 \hat{n} \cdot \vec{S}_2 \vec{v}_2 \cdot \vec{v}_2 - \frac{1}{5} \vec{S}_1 \cdot \vec{S}_2 \vec{v}_2 \cdot \vec{v}_2 \right) \Bigg) \Bigg\} \end{aligned}$$

{DiagS1S2[3, 1, 35],

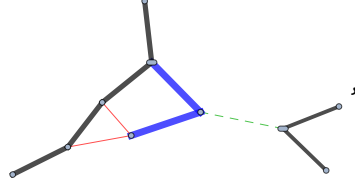

$$\begin{aligned} & G^3 m_1^2 \left( \frac{1}{r^4} \left( \frac{7}{4} \hat{n} \cdot \vec{a}_1 \hat{n} \cdot \vec{S}_1 \hat{n} \cdot \vec{S}_2 + \frac{7}{4} \hat{n} \cdot \vec{S}_1 \hat{n} \cdot \vec{v}_1 \hat{n} \cdot \vec{S}_2 - \frac{23}{100} \vec{S}_1 \cdot \vec{v}_1 \hat{n} \cdot \vec{S}_2 - \right. \right. \\ & \frac{23}{100} \vec{S}_1 \cdot \vec{a}_1 \hat{n} \cdot \vec{S}_2 + \frac{19}{4} \hat{n} \cdot \vec{S}_2 \hat{n} \cdot \vec{S}_1 \hat{n} \cdot \vec{v}_1 - \frac{3}{100} \hat{n} \cdot \vec{v}_1 \vec{S}_1 \cdot \vec{S}_2 - \frac{131}{100} \hat{n} \cdot \vec{S}_1 \vec{S}_2 \cdot \vec{v}_1 - \\ & \left. \frac{131}{100} \hat{n} \cdot \vec{v}_1 \vec{S}_1 \cdot \vec{S}_2 - \frac{3}{100} \hat{n} \cdot \vec{a}_1 \vec{S}_1 \cdot \vec{S}_2 - \frac{71}{100} \hat{n} \cdot \vec{S}_2 \vec{S}_1 \cdot \vec{v}_1 - \frac{103}{100} \hat{n} \cdot \vec{S}_1 \vec{S}_2 \cdot \vec{a}_1 - \frac{103}{100} \hat{n} \cdot \vec{S}_1 \vec{S}_2 \cdot \vec{v}_1 \right) + \\ & \frac{1}{r^5} \left( -\frac{169}{4} \hat{n} \cdot \vec{S}_1 \hat{n} \cdot \vec{S}_2 (\hat{n} \cdot \vec{v}_1)^2 + \frac{2031}{196} \vec{S}_1 \cdot \vec{S}_2 (\hat{n} \cdot \vec{v}_1)^2 + \frac{157}{4} \hat{n} \cdot \vec{S}_1 \hat{n} \cdot \vec{S}_2 \hat{n} \cdot \vec{v}_2 \hat{n} \cdot \vec{v}_1 - \right. \\ & \frac{31}{4} \hat{n} \cdot \vec{v}_2 \vec{S}_1 \cdot \vec{S}_2 \hat{n} \cdot \vec{v}_1 + \frac{1009}{98} \hat{n} \cdot \vec{S}_2 \vec{S}_1 \cdot \vec{v}_1 \hat{n} \cdot \vec{v}_1 - \frac{19}{4} \hat{n} \cdot \vec{S}_2 \vec{S}_1 \cdot \vec{v}_2 \hat{n} \cdot \vec{v}_1 + \frac{1107}{98} \hat{n} \cdot \vec{S}_1 \vec{S}_2 \cdot \vec{v}_1 \hat{n} \cdot \vec{v}_1 - \\ & \frac{19}{4} \hat{n} \cdot \vec{S}_1 \vec{S}_2 \cdot \vec{v}_2 \hat{n} \cdot \vec{v}_1 + \frac{1}{7} \hat{n} \times \vec{S}_1 \cdot \vec{v}_1 \hat{n} \times \vec{S}_2 \cdot \vec{v}_1 - \frac{19}{4} \hat{n} \cdot \vec{S}_2 \hat{n} \cdot \vec{v}_2 \vec{S}_1 \cdot \vec{v}_1 - \\ & \frac{31}{4} \hat{n} \cdot \vec{S}_1 \hat{n} \cdot \vec{v}_2 \vec{S}_2 \cdot \vec{v}_1 - \frac{4247 \vec{S}_1 \cdot \vec{v}_1 \vec{S}_2 \cdot \vec{v}_1}{2450} + \frac{131}{100} \vec{S}_1 \cdot \vec{v}_2 \vec{S}_2 \cdot \vec{v}_1 + \frac{71}{100} \vec{S}_1 \cdot \vec{v}_1 \vec{S}_2 \cdot \vec{v}_2 + \\ & \left. \frac{1093}{196} \hat{n} \cdot \vec{S}_1 \hat{n} \cdot \vec{S}_2 \vec{v}_1 \cdot \vec{v}_1 - \frac{10337 \vec{S}_1 \cdot \vec{S}_2 \vec{v}_1 \cdot \vec{v}_1}{4900} - \frac{19}{4} \hat{n} \cdot \vec{S}_1 \hat{n} \cdot \vec{S}_2 \vec{v}_1 \cdot \vec{v}_2 + \frac{131}{100} \vec{S}_1 \cdot \vec{S}_2 \vec{v}_1 \cdot \vec{v}_2 \right) + \\ & \left( \frac{1}{r^4} \left( -3 \hat{n} \cdot \vec{a}_1 \hat{n} \cdot \vec{S}_1 \hat{n} \cdot \vec{S}_2 - 3 \hat{n} \cdot \vec{S}_1 \hat{n} \cdot \vec{v}_1 \hat{n} \cdot \vec{S}_2 + \frac{3}{5} \vec{S}_1 \cdot \vec{v}_1 \hat{n} \cdot \vec{S}_2 + \frac{3}{5} \vec{S}_1 \cdot \vec{a}_1 \hat{n} \cdot \vec{S}_2 - 6 \hat{n} \cdot \vec{S}_2 \hat{n} \cdot \vec{S}_1 \hat{n} \cdot \vec{v}_1 + \frac{3}{5} \hat{n} \cdot \vec{v}_1 \vec{S}_1 \cdot \right. \right. \\ & \left. \left. \vec{S}_2 + \frac{6}{5} \hat{n} \cdot \vec{S}_1 \vec{S}_2 \cdot \vec{v}_1 + \frac{6}{5} \hat{n} \cdot \vec{v}_1 \vec{S}_1 \cdot \vec{S}_2 + \frac{3}{5} \hat{n} \cdot \vec{a}_1 \vec{S}_1 \cdot \vec{S}_2 + \frac{6}{5} \hat{n} \cdot \vec{S}_2 \vec{S}_1 \cdot \vec{v}_1 + \frac{3}{5} \hat{n} \cdot \vec{S}_1 \vec{S}_2 \cdot \vec{a}_1 + \frac{3}{5} \hat{n} \cdot \vec{S}_1 \vec{S}_2 \cdot \vec{v}_1 \right) + \right. \\ & \frac{1}{r^5} \left( \frac{87}{2} \hat{n} \cdot \vec{S}_1 \hat{n} \cdot \vec{S}_2 (\hat{n} \cdot \vec{v}_1)^2 - \frac{87}{14} \vec{S}_1 \cdot \vec{S}_2 (\hat{n} \cdot \vec{v}_1)^2 - 42 \hat{n} \cdot \vec{S}_1 \hat{n} \cdot \vec{S}_2 \hat{n} \cdot \vec{v}_2 \hat{n} \cdot \vec{v}_1 + 6 \hat{n} \cdot \vec{v}_2 \vec{S}_1 \cdot \vec{S}_2 \hat{n} \cdot \vec{v}_1 - \right. \\ & \frac{87}{7} \hat{n} \cdot \vec{S}_2 \vec{S}_1 \cdot \vec{v}_1 \hat{n} \cdot \vec{v}_1 + 6 \hat{n} \cdot \vec{S}_2 \vec{S}_1 \cdot \vec{v}_2 \hat{n} \cdot \vec{v}_1 - \frac{87}{7} \hat{n} \cdot \vec{S}_1 \vec{S}_2 \cdot \vec{v}_1 \hat{n} \cdot \vec{v}_1 + 6 \hat{n} \cdot \vec{S}_1 \vec{S}_2 \cdot \vec{v}_2 \hat{n} \cdot \vec{v}_1 + \\ & 6 \hat{n} \cdot \vec{S}_2 \hat{n} \cdot \vec{v}_2 \vec{S}_1 \cdot \vec{v}_1 + 6 \hat{n} \cdot \vec{S}_1 \hat{n} \cdot \vec{v}_2 \vec{S}_2 \cdot \vec{v}_1 + \frac{87}{35} \vec{S}_1 \cdot \vec{v}_1 \vec{S}_2 \cdot \vec{v}_1 - \frac{6}{5} \vec{S}_1 \cdot \vec{v}_2 \vec{S}_2 \cdot \vec{v}_1 - \frac{6}{5} \vec{S}_1 \cdot \vec{v}_1 \vec{S}_2 \cdot \vec{v}_2 - \\ & \left. \frac{87}{14} \hat{n} \cdot \vec{S}_1 \hat{n} \cdot \vec{S}_2 \vec{v}_1 \cdot \vec{v}_1 + \frac{87}{70} \vec{S}_1 \cdot \vec{S}_2 \vec{v}_1 \cdot \vec{v}_1 + 6 \hat{n} \cdot \vec{S}_1 \hat{n} \cdot \vec{S}_2 \vec{v}_1 \cdot \vec{v}_2 - \frac{6}{5} \vec{S}_1 \cdot \vec{S}_2 \vec{v}_1 \cdot \vec{v}_2 \right) \Bigg) \log \left( \frac{r}{R_0} \right) + \frac{1}{\epsilon_d} \\ & \left( \frac{1}{r^4} \left( \hat{n} \cdot \vec{a}_1 \hat{n} \cdot \vec{S}_1 \hat{n} \cdot \vec{S}_2 + \hat{n} \cdot \vec{S}_1 \hat{n} \cdot \vec{v}_1 \hat{n} \cdot \vec{S}_2 - \frac{1}{5} \vec{S}_1 \cdot \vec{v}_1 \hat{n} \cdot \vec{S}_2 - \frac{1}{5} \vec{S}_1 \cdot \vec{a}_1 \hat{n} \cdot \vec{S}_2 + 2 \hat{n} \cdot \vec{S}_2 \hat{n} \cdot \vec{S}_1 \hat{n} \cdot \vec{v}_1 - \frac{1}{5} \hat{n} \cdot \vec{v}_1 \vec{S}_1 \cdot \vec{S}_2 - \right. \right. \\ & \left. \left. \frac{2}{5} \hat{n} \cdot \vec{S}_1 \vec{S}_2 \cdot \vec{v}_1 - \frac{2}{5} \hat{n} \cdot \vec{v}_1 \vec{S}_1 \cdot \vec{S}_2 - \frac{1}{5} \hat{n} \cdot \vec{a}_1 \vec{S}_1 \cdot \vec{S}_2 - \frac{2}{5} \hat{n} \cdot \vec{S}_2 \vec{S}_1 \cdot \vec{v}_1 - \frac{1}{5} \hat{n} \cdot \vec{S}_1 \vec{S}_2 \cdot \vec{a}_1 - \frac{1}{5} \hat{n} \cdot \vec{S}_1 \vec{S}_2 \cdot \vec{v}_1 \right) + \frac{1}{r^5} \right. \end{aligned}$$

$$\left( -\frac{29}{2} \hat{n} \cdot \vec{S}_1 \hat{n} \cdot \vec{S}_2 (\hat{n} \cdot \vec{v}_1)^2 + \frac{29}{14} \vec{S}_1 \cdot \vec{S}_2 (\hat{n} \cdot \vec{v}_1)^2 + 14 \hat{n} \cdot \vec{S}_1 \hat{n} \cdot \vec{S}_2 \hat{n} \cdot \vec{v}_2 \hat{n} \cdot \vec{v}_1 - 2 \hat{n} \cdot \vec{v}_2 \vec{S}_1 \cdot \vec{S}_2 \hat{n} \cdot \vec{v}_1 + \right. \\ \left. \frac{29}{7} \hat{n} \cdot \vec{S}_2 \vec{S}_1 \cdot \vec{v}_1 \hat{n} \cdot \vec{v}_1 - 2 \hat{n} \cdot \vec{S}_2 \vec{S}_1 \cdot \vec{v}_2 \hat{n} \cdot \vec{v}_1 + \frac{29}{7} \hat{n} \cdot \vec{S}_1 \vec{S}_2 \cdot \vec{v}_1 \hat{n} \cdot \vec{v}_1 - 2 \hat{n} \cdot \vec{S}_1 \vec{S}_2 \cdot \vec{v}_2 \hat{n} \cdot \vec{v}_1 - \right. \\ \left. 2 \hat{n} \cdot \vec{S}_2 \hat{n} \cdot \vec{v}_2 \vec{S}_1 \cdot \vec{v}_1 - 2 \hat{n} \cdot \vec{S}_1 \hat{n} \cdot \vec{v}_2 \vec{S}_2 \cdot \vec{v}_1 - \frac{29}{35} \vec{S}_1 \cdot \vec{v}_1 \vec{S}_2 \cdot \vec{v}_1 + \frac{2}{5} \vec{S}_1 \cdot \vec{v}_2 \vec{S}_2 \cdot \vec{v}_1 + \frac{2}{5} \vec{S}_1 \cdot \vec{v}_1 \vec{S}_2 \cdot \vec{v}_2 + \right. \\ \left. \frac{29}{14} \hat{n} \cdot \vec{S}_1 \hat{n} \cdot \vec{S}_2 \vec{v}_1 \cdot \vec{v}_1 - \frac{29}{70} \vec{S}_1 \cdot \vec{S}_2 \vec{v}_1 \cdot \vec{v}_1 - 2 \hat{n} \cdot \vec{S}_1 \hat{n} \cdot \vec{S}_2 \vec{v}_1 \cdot \vec{v}_2 + \frac{2}{5} \vec{S}_1 \cdot \vec{S}_2 \vec{v}_1 \cdot \vec{v}_2 \right) \Bigg) \Bigg\}$$

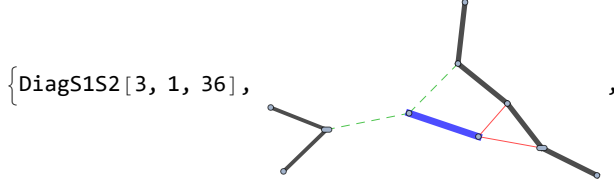

$$\frac{G^3 m_1^2 \left( -\frac{4}{7} \hat{n} \times \vec{S}_1 \cdot \vec{v}_1 \hat{n} \times \vec{S}_2 \cdot \vec{v}_1 + \frac{4}{7} \vec{S}_1 \cdot \vec{S}_2 (\hat{n} \cdot \vec{v}_1)^2 - \frac{4}{7} \hat{n} \cdot \vec{S}_1 \hat{n} \cdot \vec{v}_1 \vec{S}_2 \cdot \vec{v}_1 \right)}{r^5} \Bigg\}$$

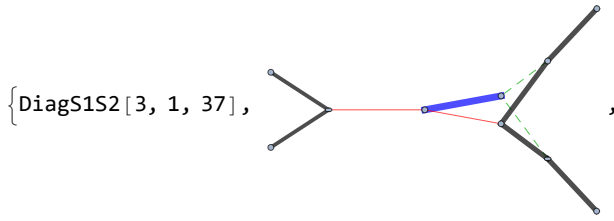

$$\frac{G^3 m_1^2 \left( 20 \hat{n} \times \vec{S}_1 \cdot \vec{v}_1 \hat{n} \times \vec{S}_2 \cdot \vec{v}_2 + 4 \vec{S}_1 \cdot \vec{v}_2 \vec{S}_2 \cdot \vec{v}_1 - 4 \vec{S}_1 \cdot \vec{S}_2 \vec{v}_1 \cdot \vec{v}_2 \right)}{r^5} \Bigg\}$$

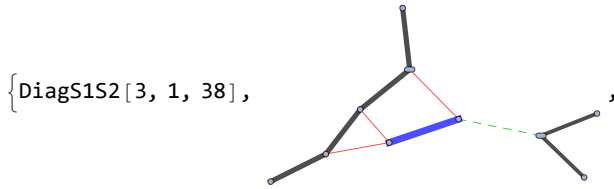

$$G^3 m_1^2 \left( \frac{-\frac{4}{5} \vec{S}_1 \cdot \vec{S}_2 \hat{n} \cdot \vec{a}_1 + \frac{4}{5} \vec{S}_2 \cdot \vec{a}_1 \hat{n} \cdot \vec{S}_1 - \frac{4}{5} \vec{S}_1 \cdot \vec{S}_2 \hat{n} \cdot \vec{v}_1 + \frac{4}{5} \hat{n} \cdot \vec{S}_1 \vec{S}_2 \cdot \vec{v}_1 - \frac{4}{5} \vec{S}_1 \cdot \vec{S}_2 \hat{n} \cdot \vec{v}_1 + \frac{4}{5} \hat{n} \cdot \vec{S}_1 \vec{S}_2 \cdot \vec{v}_1}{r^4} + \right. \\ \left. \frac{1}{r^5} \left( -\frac{18}{7} \hat{n} \times \vec{S}_1 \cdot \vec{v}_1 \hat{n} \times \vec{S}_2 \cdot \vec{v}_1 + \frac{18}{7} \vec{S}_1 \cdot \vec{S}_2 (\hat{n} \cdot \vec{v}_1)^2 - 4 \vec{S}_1 \cdot \vec{S}_2 \hat{n} \cdot \vec{v}_2 \hat{n} \cdot \vec{v}_1 - \right. \right. \\ \left. \left. \frac{18}{7} \hat{n} \cdot \vec{S}_1 \hat{n} \cdot \vec{v}_1 \vec{S}_2 \cdot \vec{v}_1 + 4 \hat{n} \cdot \vec{S}_1 \hat{n} \cdot \vec{v}_2 \vec{S}_2 \cdot \vec{v}_1 - \frac{4}{5} \vec{S}_1 \cdot \vec{v}_2 \vec{S}_2 \cdot \vec{v}_1 + \frac{4}{5} \vec{S}_1 \cdot \vec{S}_2 \vec{v}_1 \cdot \vec{v}_2 \right) \right) \Bigg\}$$

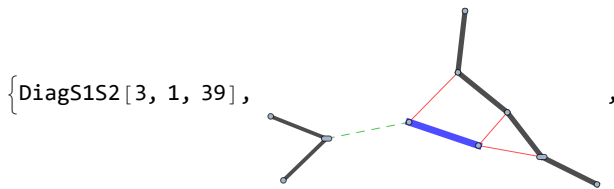

$$G^3 m_1^2 \left\{ \frac{1}{r^5} \left( -\frac{10}{7} \hat{n} \times \vec{S}_1 \cdot \vec{v}_1 \hat{n} \times \vec{S}_2 \cdot \vec{v}_1 - \frac{18}{7} \vec{S}_1 \cdot \vec{S}_2 (\hat{n} \cdot \vec{v}_1)^2 + 4 \vec{S}_1 \cdot \vec{S}_2 \hat{n} \cdot \vec{v}_2 \hat{n} \cdot \vec{v}_1 + \right. \right. \\ \left. \frac{18}{7} \hat{n} \cdot \vec{S}_1 \hat{n} \cdot \vec{v}_1 \vec{S}_2 \cdot \vec{v}_1 - 4 \hat{n} \cdot \vec{S}_1 \hat{n} \cdot \vec{v}_2 \vec{S}_2 \cdot \vec{v}_1 - \frac{4}{5} \vec{S}_1 \cdot \vec{v}_1 \vec{S}_2 \cdot \vec{v}_1 + \frac{4}{5} \vec{S}_1 \cdot \vec{v}_2 \vec{S}_2 \cdot \vec{v}_1 + \right. \\ \left. \left. \frac{4}{5} \vec{S}_1 \cdot \vec{S}_2 \vec{v}_1 \cdot \vec{v}_1 - \frac{4}{5} \vec{S}_1 \cdot \vec{S}_2 \vec{v}_1 \cdot \vec{v}_2 \right) + \frac{\frac{4}{5} \vec{S}_1 \cdot \vec{S}_2 \hat{n} \cdot \vec{v}_1 - \frac{4}{5} \hat{n} \cdot \vec{S}_1 \vec{S}_2 \cdot \vec{v}_1}{r^4} \right\}$$

{DiagS1S2 [3, 1, 40],

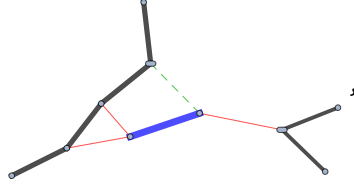

$$\frac{G^3 m_1^2 \left( 6 \hat{n} \times \vec{S}_1 \cdot \vec{v}_1 \hat{n} \times \vec{S}_2 \cdot \vec{v}_2 + \frac{6}{5} \vec{S}_1 \cdot \vec{v}_2 \vec{S}_2 \cdot \vec{v}_1 - \frac{6}{5} \vec{S}_1 \cdot \vec{S}_2 \vec{v}_1 \cdot \vec{v}_2 \right)}{r^5} \}$$

{DiagS1S2 [3, 1, 41],

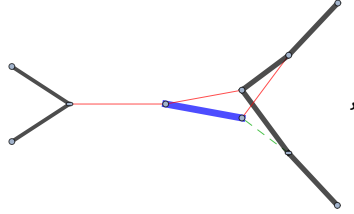

$$\frac{G^3 m_1^2 \left( -10 \hat{n} \times \vec{S}_1 \cdot \vec{v}_1 \hat{n} \times \vec{S}_2 \cdot \vec{v}_2 - 2 \vec{S}_1 \cdot \vec{v}_2 \vec{S}_2 \cdot \vec{v}_1 + 2 \vec{S}_1 \cdot \vec{S}_2 \vec{v}_1 \cdot \vec{v}_2 \right)}{r^5} \}$$

{DiagS1S2 [3, 1, 42],

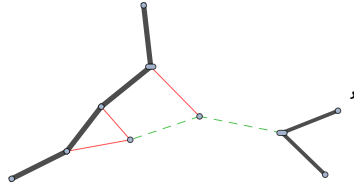

$$\frac{G^3 m_1^2 \left( -6 \hat{n} \times \vec{S}_1 \cdot \vec{v}_1 \hat{n} \times \vec{S}_2 \cdot \vec{v}_1 - 2 \vec{S}_1 \cdot \vec{S}_2 (\hat{n} \cdot \vec{v}_1)^2 + 2 \hat{n} \cdot \vec{S}_1 \hat{n} \cdot \vec{v}_1 \vec{S}_2 \cdot \vec{v}_1 - \frac{8}{5} \vec{S}_1 \cdot \vec{v}_1 \vec{S}_2 \cdot \vec{v}_1 + \frac{8}{5} \vec{S}_1 \cdot \vec{S}_2 \vec{v}_1 \cdot \vec{v}_1 \right)}{r^5} \}$$

{DiagS1S2 [3, 1, 43],

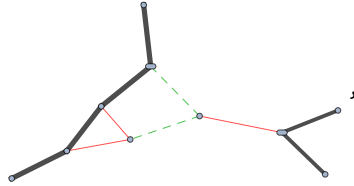

$$\frac{G^3 m_1^2 \left( 2 \hat{n} \times \vec{S}_1 \cdot \vec{v}_1 \hat{n} \times \vec{S}_2 \cdot \vec{v}_2 + \frac{2}{5} \vec{S}_1 \cdot \vec{v}_2 \vec{S}_2 \cdot \vec{v}_1 - \frac{2}{5} \vec{S}_1 \cdot \vec{S}_2 \vec{v}_1 \cdot \vec{v}_2 \right)}{r^5} \}$$

{DiagS1S2 [3, 1, 44],

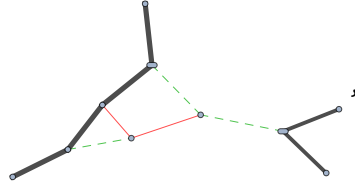

$$\begin{aligned}
 & G^3 m_1^2 \left( \frac{1}{r^4} \left( -4 \hat{n} \cdot \vec{S}_2 \hat{n} \cdot \vec{S}_1 \hat{n} \cdot \vec{v}_1 - 4 \hat{n} \cdot \vec{S}_1 \hat{n} \cdot \vec{S}_2 \hat{n} \cdot \vec{v}_1 + \frac{92}{25} \vec{S}_1 \cdot \vec{S}_2 \hat{n} \cdot \vec{v}_1 + \right. \right. \\
 & \quad \left. \frac{92}{25} \vec{S}_1 \cdot \vec{S}_2 \hat{n} \cdot \vec{v}_1 + \frac{32}{25} \hat{n} \cdot \vec{S}_2 \vec{S}_1 \cdot \vec{v}_1 - \frac{88}{25} \hat{n} \cdot \vec{S}_1 \vec{S}_2 \cdot \vec{v}_1 + \frac{32}{25} \hat{n} \cdot \vec{S}_2 \vec{S}_1 \cdot \vec{v}_1 - \frac{88}{25} \hat{n} \cdot \vec{S}_1 \vec{S}_2 \cdot \vec{v}_1 \right) + \frac{1}{r^5} \\
 & \quad \left( 48 \hat{n} \cdot \vec{S}_1 \hat{n} \cdot \vec{S}_2 (\hat{n} \cdot \vec{v}_1)^2 + \frac{432}{49} \vec{S}_1 \cdot \vec{S}_2 (\hat{n} \cdot \vec{v}_1)^2 - 16 \hat{n} \cdot \vec{S}_1 \hat{n} \cdot \vec{S}_2 \hat{n} \cdot \vec{v}_2 \hat{n} \cdot \vec{v}_1 + 16 \hat{n} \cdot \vec{v}_2 \vec{S}_1 \cdot \vec{S}_2 \hat{n} \cdot \vec{v}_1 - \right. \\
 & \quad \frac{648}{49} \hat{n} \cdot \vec{S}_2 \vec{S}_1 \cdot \vec{v}_1 \hat{n} \cdot \vec{v}_1 + 4 \hat{n} \cdot \vec{S}_2 \vec{S}_1 \cdot \vec{v}_2 \hat{n} \cdot \vec{v}_1 - \frac{1488}{49} \hat{n} \cdot \vec{S}_1 \vec{S}_2 \cdot \vec{v}_1 \hat{n} \cdot \vec{v}_1 + 4 \hat{n} \cdot \vec{S}_1 \vec{S}_2 \cdot \vec{v}_2 \hat{n} \cdot \vec{v}_1 + \\
 & \quad \frac{96}{7} \hat{n} \times \vec{S}_1 \cdot \vec{v}_1 \hat{n} \times \vec{S}_2 \cdot \vec{v}_1 + 4 \hat{n} \cdot \vec{S}_2 \hat{n} \cdot \vec{v}_2 \vec{S}_1 \cdot \vec{v}_1 - 20 \hat{n} \cdot \vec{S}_1 \hat{n} \cdot \vec{v}_2 \vec{S}_2 \cdot \vec{v}_1 + \frac{10632 \vec{S}_1 \cdot \vec{v}_1 \vec{S}_2 \cdot \vec{v}_1}{1225} + \frac{88}{25} \vec{S}_1 \cdot \vec{v}_2 \vec{S}_2 \cdot \vec{v}_1 - \\
 & \quad \left. \frac{32}{25} \vec{S}_1 \cdot \vec{v}_1 \vec{S}_2 \cdot \vec{v}_2 + \frac{684}{49} \hat{n} \cdot \vec{S}_1 \hat{n} \cdot \vec{S}_2 \vec{v}_1 \cdot \vec{v}_1 - \frac{20724 \vec{S}_1 \cdot \vec{S}_2 \vec{v}_1 \cdot \vec{v}_1}{1225} + 4 \hat{n} \cdot \vec{S}_1 \hat{n} \cdot \vec{S}_2 \vec{v}_1 \cdot \vec{v}_2 - \frac{92}{25} \vec{S}_1 \cdot \vec{S}_2 \vec{v}_1 \cdot \vec{v}_2 \right) + \\
 & \quad \left( \frac{1}{r^4} \left( -12 \hat{n} \cdot \vec{S}_2 \hat{n} \cdot \vec{S}_1 \hat{n} \cdot \vec{v}_1 - 12 \hat{n} \cdot \vec{S}_1 \hat{n} \cdot \vec{S}_2 \hat{n} \cdot \vec{v}_1 + \frac{12}{5} \vec{S}_1 \cdot \vec{S}_2 \hat{n} \cdot \vec{v}_1 + \frac{12}{5} \vec{S}_1 \cdot \vec{S}_2 \hat{n} \cdot \vec{v}_1 + \right. \right. \\
 & \quad \left. \frac{12}{5} \hat{n} \cdot \vec{S}_2 \vec{S}_1 \cdot \vec{v}_1 + \frac{12}{5} \hat{n} \cdot \vec{S}_1 \vec{S}_2 \cdot \vec{v}_1 + \frac{12}{5} \hat{n} \cdot \vec{S}_2 \vec{S}_1 \cdot \vec{v}_1 + \frac{12}{5} \hat{n} \cdot \vec{S}_1 \vec{S}_2 \cdot \vec{v}_1 \right) + \frac{1}{r^5} \\
 & \quad \left( -12 \hat{n} \cdot \vec{S}_1 \hat{n} \cdot \vec{S}_2 (\hat{n} \cdot \vec{v}_1)^2 + \frac{12}{7} \vec{S}_1 \cdot \vec{S}_2 (\hat{n} \cdot \vec{v}_1)^2 - 84 \hat{n} \cdot \vec{S}_1 \hat{n} \cdot \vec{S}_2 \hat{n} \cdot \vec{v}_2 \hat{n} \cdot \vec{v}_1 + 12 \hat{n} \cdot \vec{v}_2 \vec{S}_1 \cdot \vec{S}_2 \hat{n} \cdot \vec{v}_1 + \right. \\
 & \quad \frac{24}{7} \hat{n} \cdot \vec{S}_2 \vec{S}_1 \cdot \vec{v}_1 \hat{n} \cdot \vec{v}_1 + 12 \hat{n} \cdot \vec{S}_2 \vec{S}_1 \cdot \vec{v}_2 \hat{n} \cdot \vec{v}_1 + \frac{24}{7} \hat{n} \cdot \vec{S}_1 \vec{S}_2 \cdot \vec{v}_1 \hat{n} \cdot \vec{v}_1 + 12 \hat{n} \cdot \vec{S}_1 \vec{S}_2 \cdot \vec{v}_2 \hat{n} \cdot \vec{v}_1 + \\
 & \quad 12 \hat{n} \cdot \vec{S}_2 \hat{n} \cdot \vec{v}_2 \vec{S}_1 \cdot \vec{v}_1 + 12 \hat{n} \cdot \vec{S}_1 \hat{n} \cdot \vec{v}_2 \vec{S}_2 \cdot \vec{v}_1 - \frac{24}{35} \vec{S}_1 \cdot \vec{v}_1 \vec{S}_2 \cdot \vec{v}_1 - \frac{12}{5} \vec{S}_1 \cdot \vec{v}_2 \vec{S}_2 \cdot \vec{v}_1 - \frac{12}{5} \vec{S}_1 \cdot \vec{v}_1 \vec{S}_2 \cdot \vec{v}_2 + \\
 & \quad \left. \frac{12}{7} \hat{n} \cdot \vec{S}_1 \hat{n} \cdot \vec{S}_2 \vec{v}_1 \cdot \vec{v}_1 - \frac{12}{35} \vec{S}_1 \cdot \vec{S}_2 \vec{v}_1 \cdot \vec{v}_1 + 12 \hat{n} \cdot \vec{S}_1 \hat{n} \cdot \vec{S}_2 \vec{v}_1 \cdot \vec{v}_2 - \frac{12}{5} \vec{S}_1 \cdot \vec{S}_2 \vec{v}_1 \cdot \vec{v}_2 \right) \log \left( \frac{r}{R_0} \right) + \\
 & \quad \frac{1}{\epsilon_d} \left( \frac{1}{r^4} \left( 4 \hat{n} \cdot \vec{S}_2 \hat{n} \cdot \vec{S}_1 \hat{n} \cdot \vec{v}_1 + 4 \hat{n} \cdot \vec{S}_1 \hat{n} \cdot \vec{S}_2 \hat{n} \cdot \vec{v}_1 - \frac{4}{5} \vec{S}_1 \cdot \vec{S}_2 \hat{n} \cdot \vec{v}_1 - \frac{4}{5} \vec{S}_1 \cdot \vec{S}_2 \hat{n} \cdot \vec{v}_1 - \right. \right. \\
 & \quad \left. \frac{4}{5} \hat{n} \cdot \vec{S}_2 \vec{S}_1 \cdot \vec{v}_1 - \frac{4}{5} \hat{n} \cdot \vec{S}_1 \vec{S}_2 \cdot \vec{v}_1 - \frac{4}{5} \hat{n} \cdot \vec{S}_2 \vec{S}_1 \cdot \vec{v}_1 - \frac{4}{5} \hat{n} \cdot \vec{S}_1 \vec{S}_2 \cdot \vec{v}_1 \right) + \frac{1}{r^5} \\
 & \quad \left( 4 \hat{n} \cdot \vec{S}_1 \hat{n} \cdot \vec{S}_2 (\hat{n} \cdot \vec{v}_1)^2 - \frac{4}{7} \vec{S}_1 \cdot \vec{S}_2 (\hat{n} \cdot \vec{v}_1)^2 + 28 \hat{n} \cdot \vec{S}_1 \hat{n} \cdot \vec{S}_2 \hat{n} \cdot \vec{v}_2 \hat{n} \cdot \vec{v}_1 - 4 \hat{n} \cdot \vec{v}_2 \vec{S}_1 \cdot \vec{S}_2 \hat{n} \cdot \vec{v}_1 - \right. \\
 & \quad \frac{8}{7} \hat{n} \cdot \vec{S}_2 \vec{S}_1 \cdot \vec{v}_1 \hat{n} \cdot \vec{v}_1 - 4 \hat{n} \cdot \vec{S}_2 \vec{S}_1 \cdot \vec{v}_2 \hat{n} \cdot \vec{v}_1 - \frac{8}{7} \hat{n} \cdot \vec{S}_1 \vec{S}_2 \cdot \vec{v}_1 \hat{n} \cdot \vec{v}_1 - 4 \hat{n} \cdot \vec{S}_1 \vec{S}_2 \cdot \vec{v}_2 \hat{n} \cdot \vec{v}_1 - \\
 & \quad 4 \hat{n} \cdot \vec{S}_2 \hat{n} \cdot \vec{v}_2 \vec{S}_1 \cdot \vec{v}_1 - 4 \hat{n} \cdot \vec{S}_1 \hat{n} \cdot \vec{v}_2 \vec{S}_2 \cdot \vec{v}_1 + \frac{8}{35} \vec{S}_1 \cdot \vec{v}_1 \vec{S}_2 \cdot \vec{v}_1 + \frac{4}{5} \vec{S}_1 \cdot \vec{v}_2 \vec{S}_2 \cdot \vec{v}_1 + \frac{4}{5} \vec{S}_1 \cdot \vec{v}_1 \vec{S}_2 \cdot \vec{v}_2 - \\
 & \quad \left. \left. \frac{4}{7} \hat{n} \cdot \vec{S}_1 \hat{n} \cdot \vec{S}_2 \vec{v}_1 \cdot \vec{v}_1 + \frac{4}{35} \vec{S}_1 \cdot \vec{S}_2 \vec{v}_1 \cdot \vec{v}_1 - 4 \hat{n} \cdot \vec{S}_1 \hat{n} \cdot \vec{S}_2 \vec{v}_1 \cdot \vec{v}_2 + \frac{4}{5} \vec{S}_1 \cdot \vec{S}_2 \vec{v}_1 \cdot \vec{v}_2 \right) \right) \right) \Bigg\}
 \end{aligned}$$

{DiagS1S2 [3, 1, 45],

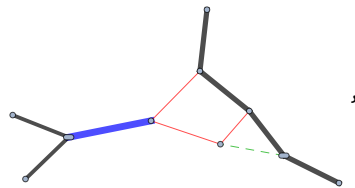



$$\frac{G^3 m_1^2 \left( \frac{4}{7} \hat{n} \times \vec{S}_1 \cdot \vec{v}_1 \hat{n} \times \vec{S}_2 \cdot \vec{v}_2 - \frac{1}{14} \vec{S}_1 \cdot \vec{S}_2 \hat{n} \cdot \vec{v}_1 \hat{n} \cdot \vec{v}_2 + \frac{1}{14} \hat{n} \cdot \vec{S}_1 \hat{n} \cdot \vec{v}_2 \vec{S}_2 \cdot \vec{v}_1 + \frac{1}{10} \vec{S}_1 \cdot \vec{v}_2 \vec{S}_2 \cdot \vec{v}_1 - \frac{1}{10} \vec{S}_1 \cdot \vec{S}_2 \vec{v}_1 \cdot \vec{v}_2 \right)}{r^5} \Bigg\}$$

{DiagS1S2 [3, 1, 46],

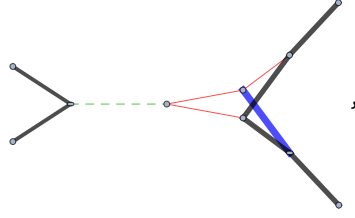

,

$$G^3 m_1^2 \left( \frac{\frac{1}{10} \vec{S}_1 \cdot \vec{S}_2 \hat{n} \cdot \vec{a}_1 - \frac{1}{10} \vec{S}_2 \cdot \vec{a}_1 \hat{n} \cdot \vec{S}_1 + \frac{1}{10} \vec{S}_1 \cdot \vec{S}_2 \hat{n} \cdot \vec{v}_1 - \frac{1}{10} \hat{n} \cdot \vec{S}_1 \vec{S}_2 \cdot \vec{v}_1}{r^4} + \right.$$

$$\left. \frac{\frac{4}{7} \hat{n} \times \vec{S}_1 \cdot \vec{v}_1 \hat{n} \times \vec{S}_2 \cdot \vec{v}_1 - \frac{1}{14} \vec{S}_1 \cdot \vec{S}_2 (\hat{n} \cdot \vec{v}_1)^2 + \frac{1}{14} \hat{n} \cdot \vec{S}_1 \hat{n} \cdot \vec{v}_1 \vec{S}_2 \cdot \vec{v}_1 + \frac{1}{10} \vec{S}_1 \cdot \vec{v}_1 \vec{S}_2 \cdot \vec{v}_1 - \frac{1}{10} \vec{S}_1 \cdot \vec{S}_2 \vec{v}_1 \cdot \vec{v}_1}{r^5} \right\}$$

{DiagS1S2 [3, 1, 47],

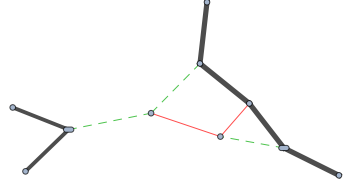

,

$$\frac{G^3 m_1^2 \left( 6 \hat{n} \times \vec{S}_1 \cdot \vec{v}_1 \hat{n} \times \vec{S}_2 \cdot \vec{v}_1 + 2 \vec{S}_1 \cdot \vec{S}_2 (\hat{n} \cdot \vec{v}_1)^2 - 2 \hat{n} \cdot \vec{S}_1 \hat{n} \cdot \vec{v}_1 \vec{S}_2 \cdot \vec{v}_1 + \frac{8}{5} \vec{S}_1 \cdot \vec{v}_1 \vec{S}_2 \cdot \vec{v}_1 - \frac{8}{5} \vec{S}_1 \cdot \vec{S}_2 \vec{v}_1 \cdot \vec{v}_1 \right)}{r^5} \Bigg\}$$

{DiagS1S2 [3, 1, 48],

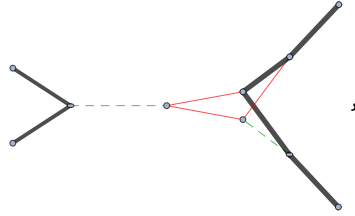

,

$$G^3 m_1^2 \left( \frac{-\frac{1}{10} \vec{S}_1 \cdot \vec{S}_2 \hat{n} \cdot \vec{a}_1 + \frac{1}{10} \vec{S}_2 \cdot \vec{a}_1 \hat{n} \cdot \vec{S}_1 - \frac{1}{10} \vec{S}_1 \cdot \vec{S}_2 \hat{n} \cdot \vec{v}_1 + \frac{1}{10} \hat{n} \cdot \vec{S}_1 \vec{S}_2 \cdot \vec{v}_1}{r^4} + \right.$$

$$\left. \frac{-\frac{4}{7} \hat{n} \times \vec{S}_1 \cdot \vec{v}_1 \hat{n} \times \vec{S}_2 \cdot \vec{v}_1 + \frac{1}{14} \vec{S}_1 \cdot \vec{S}_2 (\hat{n} \cdot \vec{v}_1)^2 - \frac{1}{14} \hat{n} \cdot \vec{S}_1 \hat{n} \cdot \vec{v}_1 \vec{S}_2 \cdot \vec{v}_1 - \frac{1}{10} \vec{S}_1 \cdot \vec{v}_1 \vec{S}_2 \cdot \vec{v}_1 + \frac{1}{10} \vec{S}_1 \cdot \vec{S}_2 \vec{v}_1 \cdot \vec{v}_1}{r^5} \right\}$$

{DiagS1S2 [3, 1, 49],

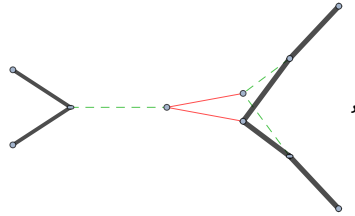

,

$$G^3 m_1^2 \left( \frac{-\frac{2}{5} \vec{S}_1 \cdot \vec{S}_2 \hat{n} \cdot \vec{a}_1 + \frac{2}{5} \vec{S}_2 \cdot \vec{a}_1 \hat{n} \cdot \vec{S}_1 - \frac{2}{5} \vec{S}_1 \cdot \vec{S}_2 \hat{n} \cdot \vec{v}_1 + \frac{2}{5} \hat{n} \cdot \vec{S}_1 \vec{S}_2 \cdot \vec{v}_1}{r^4} + \frac{-\frac{16}{7} \hat{n} \times \vec{S}_1 \cdot \vec{v}_1 \hat{n} \times \vec{S}_2 \cdot \vec{v}_1 + \frac{2}{7} \vec{S}_1 \cdot \vec{S}_2 (\hat{n} \cdot \vec{v}_1)^2 - \frac{2}{7} \hat{n} \cdot \vec{S}_1 \hat{n} \cdot \vec{v}_1 \vec{S}_2 \cdot \vec{v}_1 - \frac{2}{5} \vec{S}_1 \cdot \vec{v}_1 \vec{S}_2 \cdot \vec{v}_1 + \frac{2}{5} \vec{S}_1 \cdot \vec{S}_2 \vec{v}_1 \cdot \vec{v}_1}{r^5} \right) \Bigg\}$$

{DiagS1S2 [3, 1, 50],

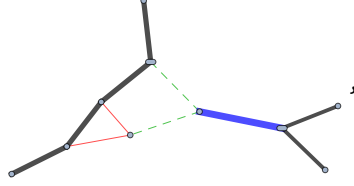

$$G^3 m_1^2 \left( \frac{1}{r^5 \in_d} \left( -\frac{3}{2} \hat{n} \cdot \vec{S}_1 \hat{n} \cdot \vec{S}_2 \hat{n} \cdot \vec{v}_1 \hat{n} \cdot \vec{v}_2 + \frac{3}{14} \hat{n} \cdot \vec{v}_1 \vec{S}_1 \cdot \vec{S}_2 \hat{n} \cdot \vec{v}_2 + \frac{3}{14} \hat{n} \cdot \vec{S}_2 \vec{S}_1 \cdot \vec{v}_1 \hat{n} \cdot \vec{v}_2 + \frac{3}{14} \hat{n} \cdot \vec{S}_1 \vec{S}_2 \cdot \vec{v}_1 \hat{n} \cdot \vec{v}_2 + \frac{3}{14} \hat{n} \cdot \vec{S}_2 \hat{n} \cdot \vec{v}_1 \vec{S}_1 \cdot \vec{v}_2 - \frac{3}{70} \vec{S}_1 \cdot \vec{v}_2 \vec{S}_2 \cdot \vec{v}_1 + \frac{3}{14} \hat{n} \cdot \vec{S}_1 \hat{n} \cdot \vec{v}_1 \vec{S}_2 \cdot \vec{v}_2 - \frac{3}{70} \vec{S}_1 \cdot \vec{v}_1 \vec{S}_2 \cdot \vec{v}_2 + \frac{3}{14} \hat{n} \cdot \vec{S}_1 \hat{n} \cdot \vec{S}_2 \vec{v}_1 \cdot \vec{v}_2 - \frac{3}{70} \vec{S}_1 \cdot \vec{S}_2 \vec{v}_1 \cdot \vec{v}_2 \right) + \frac{1}{r^5} \left( \frac{5}{7} \hat{n} \times \vec{S}_1 \cdot \vec{v}_2 \hat{n} \times \vec{S}_2 \cdot \vec{v}_1 - \frac{4}{7} \hat{n} \times \vec{S}_1 \cdot \vec{v}_1 \hat{n} \times \vec{S}_2 \cdot \vec{v}_2 - 5 \hat{n} \cdot \vec{S}_1 \hat{n} \cdot \vec{S}_2 \hat{n} \cdot \vec{v}_1 \hat{n} \cdot \vec{v}_2 + \frac{201}{98} \hat{n} \cdot \vec{v}_1 \hat{n} \cdot \vec{v}_2 \vec{S}_1 \cdot \vec{S}_2 + \frac{61}{98} \hat{n} \cdot \vec{S}_2 \hat{n} \cdot \vec{v}_2 \vec{S}_1 \cdot \vec{v}_1 + \frac{61}{98} \hat{n} \cdot \vec{S}_2 \hat{n} \cdot \vec{v}_1 \vec{S}_1 \cdot \vec{v}_2 - \frac{8}{49} \hat{n} \cdot \vec{S}_1 \hat{n} \cdot \vec{v}_2 \vec{S}_2 \cdot \vec{v}_1 - \frac{137}{2450} \vec{S}_1 \cdot \vec{v}_2 \vec{S}_2 \cdot \vec{v}_1 + \frac{61}{98} \hat{n} \cdot \vec{S}_1 \hat{n} \cdot \vec{v}_1 \vec{S}_2 \cdot \vec{v}_2 + \frac{54}{1225} \vec{S}_1 \cdot \vec{v}_1 \vec{S}_2 \cdot \vec{v}_2 - \frac{9}{98} \hat{n} \cdot \vec{S}_1 \hat{n} \cdot \vec{S}_2 \vec{v}_1 \cdot \vec{v}_2 + \frac{19}{1225} \vec{S}_1 \cdot \vec{S}_2 \vec{v}_1 \cdot \vec{v}_2 \right) + \frac{1}{r^5} \left( \frac{9}{2} \hat{n} \cdot \vec{S}_1 \hat{n} \cdot \vec{S}_2 \hat{n} \cdot \vec{v}_1 \hat{n} \cdot \vec{v}_2 - \frac{9}{14} \hat{n} \cdot \vec{v}_1 \vec{S}_1 \cdot \vec{S}_2 \hat{n} \cdot \vec{v}_2 - \frac{9}{14} \hat{n} \cdot \vec{S}_2 \vec{S}_1 \cdot \vec{v}_1 \hat{n} \cdot \vec{v}_2 - \frac{9}{14} \hat{n} \cdot \vec{S}_1 \vec{S}_2 \cdot \vec{v}_1 \hat{n} \cdot \vec{v}_2 - \frac{9}{14} \hat{n} \cdot \vec{S}_2 \hat{n} \cdot \vec{v}_1 \vec{S}_1 \cdot \vec{v}_2 + \frac{9}{70} \vec{S}_1 \cdot \vec{v}_2 \vec{S}_2 \cdot \vec{v}_1 - \frac{9}{14} \hat{n} \cdot \vec{S}_1 \hat{n} \cdot \vec{v}_1 \vec{S}_2 \cdot \vec{v}_2 + \frac{9}{70} \vec{S}_1 \cdot \vec{v}_1 \vec{S}_2 \cdot \vec{v}_2 - \frac{9}{14} \hat{n} \cdot \vec{S}_1 \hat{n} \cdot \vec{S}_2 \vec{v}_1 \cdot \vec{v}_2 + \frac{9}{70} \vec{S}_1 \cdot \vec{S}_2 \vec{v}_1 \cdot \vec{v}_2 \right) \log \left( \frac{r}{R_0} \right) \right) \Bigg\}$$

{DiagS1S2 [3, 1, 51],

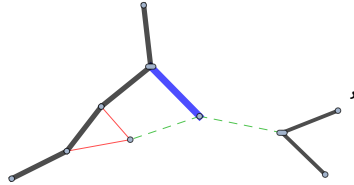

$$G^3 m_1^2 \left( \frac{1}{r^5 \in_d} \left( \frac{7}{2} \hat{n} \cdot \vec{S}_1 \hat{n} \cdot \vec{S}_2 (\hat{n} \cdot \vec{v}_1)^2 - \frac{1}{2} \vec{S}_1 \cdot \vec{S}_2 (\hat{n} \cdot \vec{v}_1)^2 - \hat{n} \cdot \vec{S}_2 \hat{n} \cdot \vec{v}_1 \vec{S}_1 \cdot \vec{v}_1 - \hat{n} \cdot \vec{S}_1 \hat{n} \cdot \vec{v}_1 \vec{S}_2 \cdot \vec{v}_1 - \frac{1}{2} \vec{v}_1 \cdot \vec{v}_1 \hat{n} \cdot \vec{S}_1 \hat{n} \cdot \vec{S}_2 + \frac{1}{5} \vec{S}_1 \cdot \vec{v}_1 \vec{S}_2 \cdot \vec{v}_1 + \frac{1}{10} \vec{S}_1 \cdot \vec{S}_2 \vec{v}_1 \cdot \vec{v}_1 \right) + \frac{1}{r^5} \log \left( \frac{r}{R_0} \right) \left( -\frac{21}{2} \hat{n} \cdot \vec{S}_1 \hat{n} \cdot \vec{S}_2 (\hat{n} \cdot \vec{v}_1)^2 + \frac{3}{2} \vec{S}_1 \cdot \vec{S}_2 (\hat{n} \cdot \vec{v}_1)^2 + 3 \hat{n} \cdot \vec{S}_2 \hat{n} \cdot \vec{v}_1 \vec{S}_1 \cdot \vec{v}_1 + 3 \hat{n} \cdot \vec{S}_1 \hat{n} \cdot \vec{v}_1 \vec{S}_2 \cdot \vec{v}_1 + \frac{3}{2} \vec{v}_1 \cdot \vec{v}_1 \hat{n} \cdot \vec{S}_1 \hat{n} \cdot \vec{S}_2 - \frac{3}{5} \vec{S}_1 \cdot \vec{v}_1 \vec{S}_2 \cdot \vec{v}_1 - \frac{3}{10} \vec{S}_1 \cdot \vec{S}_2 \vec{v}_1 \cdot \vec{v}_1 \right) + \frac{1}{r^5} \left( 3 \hat{n} \times \vec{S}_1 \cdot \vec{v}_1 \hat{n} \times \vec{S}_2 \cdot \vec{v}_1 + 12 \hat{n} \cdot \vec{S}_1 \hat{n} \cdot \vec{S}_2 (\hat{n} \cdot \vec{v}_1)^2 - 3 \vec{S}_1 \cdot \vec{S}_2 (\hat{n} \cdot \vec{v}_1)^2 - 3 \hat{n} \cdot \vec{S}_2 \hat{n} \cdot \vec{v}_1 \vec{S}_1 \cdot \vec{v}_1 - 3 \hat{n} \cdot \vec{S}_1 \hat{n} \cdot \vec{v}_1 \vec{S}_2 \cdot \vec{v}_1 + \frac{1}{2} \vec{v}_1 \cdot \vec{v}_1 \hat{n} \cdot \vec{S}_1 \hat{n} \cdot \vec{S}_2 + \frac{27}{25} \vec{S}_1 \cdot \vec{v}_1 \vec{S}_2 \cdot \vec{v}_1 - \frac{63}{50} \vec{S}_1 \cdot \vec{S}_2 \vec{v}_1 \cdot \vec{v}_1 \right) \right) \Bigg\}$$

{DiagS1S2[3, 1, 52],

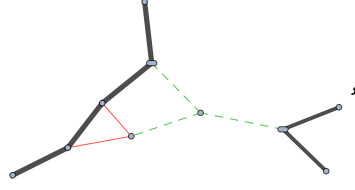

$$\begin{aligned}
 & G^3 m_1^2 \left( \frac{1}{r^4} \left( 4 \hat{n} \cdot \vec{a}_1 \hat{n} \cdot \vec{S}_1 \hat{n} \cdot \vec{S}_2 - \frac{1}{2} \hat{n} \cdot \vec{S}_1 \hat{n} \cdot \vec{v}_1 \hat{n} \cdot \vec{S}_2 + \frac{11}{50} \vec{S}_1 \cdot \vec{v}_1 \hat{n} \cdot \vec{S}_2 - \right. \right. \\
 & \quad \frac{17}{25} \vec{S}_1 \cdot \vec{a}_1 \hat{n} \cdot \vec{S}_2 - \hat{n} \cdot \vec{S}_2 \hat{n} \cdot \vec{S}_1 \hat{n} \cdot \vec{v}_1 - \frac{7}{25} \hat{n} \cdot \vec{v}_1 \vec{S}_1 \cdot \vec{S}_2 + \frac{12}{25} \hat{n} \cdot \vec{S}_1 \vec{S}_2 \cdot \vec{v}_1 + \frac{7}{25} \hat{n} \cdot \vec{v}_1 \vec{S}_1 \cdot \vec{S}_2 - \\
 & \quad \left. \frac{59}{50} \hat{n} \cdot \vec{a}_1 \vec{S}_1 \cdot \vec{S}_2 + \frac{2}{25} \hat{n} \cdot \vec{S}_2 \vec{S}_1 \cdot \vec{v}_1 - \frac{39}{50} \hat{n} \cdot \vec{S}_1 \vec{S}_2 \cdot \vec{a}_1 + \frac{3}{25} \hat{n} \cdot \vec{S}_1 \vec{S}_2 \cdot \vec{v}_1 \right) + \frac{1}{r^5} \\
 & \quad \left( -18 \hat{n} \cdot \vec{S}_1 \hat{n} \cdot \vec{S}_2 (\hat{n} \cdot \vec{v}_1)^2 + \frac{237}{49} \vec{S}_1 \cdot \vec{S}_2 (\hat{n} \cdot \vec{v}_1)^2 - 10 \hat{n} \cdot \vec{S}_1 \hat{n} \cdot \vec{S}_2 \hat{n} \cdot \vec{v}_2 \hat{n} \cdot \vec{v}_1 + 2 \hat{n} \cdot \vec{v}_2 \vec{S}_1 \cdot \vec{S}_2 \hat{n} \cdot \vec{v}_1 + \right. \\
 & \quad \frac{201}{49} \hat{n} \cdot \vec{S}_2 \vec{S}_1 \cdot \vec{v}_1 \hat{n} \cdot \vec{v}_1 + \hat{n} \cdot \vec{S}_2 \vec{S}_1 \cdot \vec{v}_2 \hat{n} \cdot \vec{v}_1 + \frac{243}{49} \hat{n} \cdot \vec{S}_1 \vec{S}_2 \cdot \vec{v}_1 \hat{n} \cdot \vec{v}_1 + \hat{n} \cdot \vec{S}_1 \vec{S}_2 \cdot \vec{v}_2 \hat{n} \cdot \vec{v}_1 - \\
 & \quad \frac{31}{14} \hat{n} \times \vec{S}_1 \cdot \vec{v}_1 \hat{n} \times \vec{S}_2 \cdot \vec{v}_1 + \hat{n} \cdot \vec{S}_2 \hat{n} \cdot \vec{v}_2 \vec{S}_1 \cdot \vec{v}_1 + 3 \hat{n} \cdot \vec{S}_1 \hat{n} \cdot \vec{v}_2 \vec{S}_2 \cdot \vec{v}_1 - \frac{2801 \vec{S}_1 \cdot \vec{v}_1 \vec{S}_2 \cdot \vec{v}_1}{2450} - \frac{12}{25} \vec{S}_1 \cdot \vec{v}_2 \vec{S}_2 \cdot \vec{v}_1 - \\
 & \quad \left. \frac{2}{25} \vec{S}_1 \cdot \vec{v}_1 \vec{S}_2 \cdot \vec{v}_2 + \frac{327}{98} \hat{n} \cdot \vec{S}_1 \hat{n} \cdot \vec{S}_2 \vec{v}_1 \cdot \vec{v}_1 - \frac{1409 \vec{S}_1 \cdot \vec{S}_2 \vec{v}_1 \cdot \vec{v}_1}{1225} + \hat{n} \cdot \vec{S}_1 \hat{n} \cdot \vec{S}_2 \vec{v}_1 \cdot \vec{v}_2 - \frac{7}{25} \vec{S}_1 \cdot \vec{S}_2 \vec{v}_1 \cdot \vec{v}_2 \right) + \\
 & \quad \left( \frac{1}{r^4} \left( -3 \hat{n} \cdot \vec{a}_1 \hat{n} \cdot \vec{S}_1 \hat{n} \cdot \vec{S}_2 - 3 \hat{n} \cdot \vec{S}_1 \hat{n} \cdot \vec{v}_1 \hat{n} \cdot \vec{S}_2 + \frac{3}{5} \vec{S}_1 \cdot \vec{v}_1 \hat{n} \cdot \vec{S}_2 + \frac{3}{5} \vec{S}_1 \cdot \vec{a}_1 \hat{n} \cdot \vec{S}_2 + 3 \hat{n} \cdot \vec{S}_2 \hat{n} \cdot \vec{S}_1 \hat{n} \cdot \vec{v}_1 + \frac{3}{5} \hat{n} \cdot \vec{v}_1 \vec{S}_1 \cdot \right. \right. \\
 & \quad \left. \vec{S}_2 - \frac{3}{5} \hat{n} \cdot \vec{S}_1 \vec{S}_2 \cdot \vec{v}_1 - \frac{3}{5} \hat{n} \cdot \vec{v}_1 \vec{S}_1 \cdot \vec{S}_2 + \frac{3}{5} \hat{n} \cdot \vec{a}_1 \vec{S}_1 \cdot \vec{S}_2 - \frac{3}{5} \hat{n} \cdot \vec{S}_2 \vec{S}_1 \cdot \vec{v}_1 + \frac{3}{5} \hat{n} \cdot \vec{S}_1 \vec{S}_2 \cdot \vec{a}_1 + \frac{3}{5} \hat{n} \cdot \vec{S}_1 \vec{S}_2 \cdot \vec{v}_1 \right) + \\
 & \quad \frac{1}{r^5} \left( \frac{51}{2} \hat{n} \cdot \vec{S}_1 \hat{n} \cdot \vec{S}_2 (\hat{n} \cdot \vec{v}_1)^2 - \frac{51}{14} \vec{S}_1 \cdot \vec{S}_2 (\hat{n} \cdot \vec{v}_1)^2 + 21 \hat{n} \cdot \vec{S}_1 \hat{n} \cdot \vec{S}_2 \hat{n} \cdot \vec{v}_2 \hat{n} \cdot \vec{v}_1 - 3 \hat{n} \cdot \vec{v}_2 \vec{S}_1 \cdot \vec{S}_2 \hat{n} \cdot \vec{v}_1 - \right. \\
 & \quad \frac{51}{7} \hat{n} \cdot \vec{S}_2 \vec{S}_1 \cdot \vec{v}_1 \hat{n} \cdot \vec{v}_1 - 3 \hat{n} \cdot \vec{S}_2 \vec{S}_1 \cdot \vec{v}_2 \hat{n} \cdot \vec{v}_1 - \frac{51}{7} \hat{n} \cdot \vec{S}_1 \vec{S}_2 \cdot \vec{v}_1 \hat{n} \cdot \vec{v}_1 - 3 \hat{n} \cdot \vec{S}_1 \vec{S}_2 \cdot \vec{v}_2 \hat{n} \cdot \vec{v}_1 - \\
 & \quad 3 \hat{n} \cdot \vec{S}_2 \hat{n} \cdot \vec{v}_2 \vec{S}_1 \cdot \vec{v}_1 - 3 \hat{n} \cdot \vec{S}_1 \hat{n} \cdot \vec{v}_2 \vec{S}_2 \cdot \vec{v}_1 + \frac{51}{35} \vec{S}_1 \cdot \vec{v}_1 \vec{S}_2 \cdot \vec{v}_1 + \frac{3}{5} \vec{S}_1 \cdot \vec{v}_2 \vec{S}_2 \cdot \vec{v}_1 + \frac{3}{5} \vec{S}_1 \cdot \vec{v}_1 \vec{S}_2 \cdot \vec{v}_2 - \\
 & \quad \left. \frac{51}{14} \hat{n} \cdot \vec{S}_1 \hat{n} \cdot \vec{S}_2 \vec{v}_1 \cdot \vec{v}_1 + \frac{51}{70} \vec{S}_1 \cdot \vec{S}_2 \vec{v}_1 \cdot \vec{v}_1 - 3 \hat{n} \cdot \vec{S}_1 \hat{n} \cdot \vec{S}_2 \vec{v}_1 \cdot \vec{v}_2 + \frac{3}{5} \vec{S}_1 \cdot \vec{S}_2 \vec{v}_1 \cdot \vec{v}_2 \right) \log \left( \frac{r}{R_0} \right) + \frac{1}{\epsilon_d} \\
 & \quad \left( \frac{1}{r^4} \left( \hat{n} \cdot \vec{a}_1 \hat{n} \cdot \vec{S}_1 \hat{n} \cdot \vec{S}_2 + \hat{n} \cdot \vec{S}_1 \hat{n} \cdot \vec{v}_1 \hat{n} \cdot \vec{S}_2 - \frac{1}{5} \vec{S}_1 \cdot \vec{v}_1 \hat{n} \cdot \vec{S}_2 - \frac{1}{5} \vec{S}_1 \cdot \vec{a}_1 \hat{n} \cdot \vec{S}_2 - \hat{n} \cdot \vec{S}_2 \hat{n} \cdot \vec{S}_1 \hat{n} \cdot \vec{v}_1 - \frac{1}{5} \hat{n} \cdot \vec{v}_1 \vec{S}_1 \cdot \vec{S}_2 + \right. \right. \\
 & \quad \left. \frac{1}{5} \hat{n} \cdot \vec{S}_1 \vec{S}_2 \cdot \vec{v}_1 + \frac{1}{5} \hat{n} \cdot \vec{v}_1 \vec{S}_1 \cdot \vec{S}_2 - \frac{1}{5} \hat{n} \cdot \vec{a}_1 \vec{S}_1 \cdot \vec{S}_2 + \frac{1}{5} \hat{n} \cdot \vec{S}_2 \vec{S}_1 \cdot \vec{v}_1 - \frac{1}{5} \hat{n} \cdot \vec{S}_1 \vec{S}_2 \cdot \vec{a}_1 - \frac{1}{5} \hat{n} \cdot \vec{S}_1 \vec{S}_2 \cdot \vec{v}_1 \right) + \\
 & \quad \frac{1}{r^5} \left( -\frac{17}{2} \hat{n} \cdot \vec{S}_1 \hat{n} \cdot \vec{S}_2 (\hat{n} \cdot \vec{v}_1)^2 + \frac{17}{14} \vec{S}_1 \cdot \vec{S}_2 (\hat{n} \cdot \vec{v}_1)^2 - 7 \hat{n} \cdot \vec{S}_1 \hat{n} \cdot \vec{S}_2 \hat{n} \cdot \vec{v}_2 \hat{n} \cdot \vec{v}_1 + \hat{n} \cdot \vec{v}_2 \vec{S}_1 \cdot \vec{S}_2 \hat{n} \cdot \vec{v}_1 + \right. \\
 & \quad \frac{17}{7} \hat{n} \cdot \vec{S}_2 \vec{S}_1 \cdot \vec{v}_1 \hat{n} \cdot \vec{v}_1 + \hat{n} \cdot \vec{S}_2 \vec{S}_1 \cdot \vec{v}_2 \hat{n} \cdot \vec{v}_1 + \frac{17}{7} \hat{n} \cdot \vec{S}_1 \vec{S}_2 \cdot \vec{v}_1 \hat{n} \cdot \vec{v}_1 + \hat{n} \cdot \vec{S}_1 \vec{S}_2 \cdot \vec{v}_2 \hat{n} \cdot \vec{v}_1 + \\
 & \quad \hat{n} \cdot \vec{S}_2 \hat{n} \cdot \vec{v}_2 \vec{S}_1 \cdot \vec{v}_1 + \hat{n} \cdot \vec{S}_1 \hat{n} \cdot \vec{v}_2 \vec{S}_2 \cdot \vec{v}_1 - \frac{17}{35} \vec{S}_1 \cdot \vec{v}_1 \vec{S}_2 \cdot \vec{v}_1 - \frac{1}{5} \vec{S}_1 \cdot \vec{v}_2 \vec{S}_2 \cdot \vec{v}_1 - \frac{1}{5} \vec{S}_1 \cdot \vec{v}_1 \vec{S}_2 \cdot \vec{v}_2 + \\
 & \quad \left. \left. \frac{17}{14} \hat{n} \cdot \vec{S}_1 \hat{n} \cdot \vec{S}_2 \vec{v}_1 \cdot \vec{v}_1 - \frac{17}{70} \vec{S}_1 \cdot \vec{S}_2 \vec{v}_1 \cdot \vec{v}_1 + \hat{n} \cdot \vec{S}_1 \hat{n} \cdot \vec{S}_2 \vec{v}_1 \cdot \vec{v}_2 - \frac{1}{5} \vec{S}_1 \cdot \vec{S}_2 \vec{v}_1 \cdot \vec{v}_2 \right) \right) \Bigg\}
 \end{aligned}$$

{DiagS1S2 [3, 1, 53],

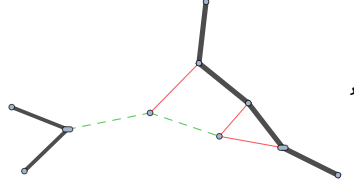

$$G^3 m_1^2 \left\{ \frac{-4 \vec{S}_1 \cdot \vec{S}_2 \hat{n} \cdot \vec{a}_1 + 4 \vec{S}_2 \cdot \vec{a}_1 \hat{n} \cdot \vec{S}_1 - 4 \vec{S}_1 \cdot \vec{S}_2 \hat{n} \cdot \vec{v}_1 + 4 \hat{n} \cdot \vec{S}_1 \vec{S}_2 \cdot \vec{v}_1}{r^4} + \frac{-14 \hat{n} \times \vec{S}_1 \cdot \vec{v}_1 \hat{n} \times \vec{S}_2 \cdot \vec{v}_1 + 2 \vec{S}_1 \cdot \vec{S}_2 (\hat{n} \cdot \vec{v}_1)^2 - 2 \hat{n} \cdot \vec{S}_1 \hat{n} \cdot \vec{v}_1 \vec{S}_2 \cdot \vec{v}_1 - \frac{12}{5} \vec{S}_1 \cdot \vec{v}_1 \vec{S}_2 \cdot \vec{v}_1 + \frac{12}{5} \vec{S}_1 \cdot \vec{S}_2 \vec{v}_1 \cdot \vec{v}_1}{r^5} \right\}$$

{DiagS1S2 [3, 1, 54],

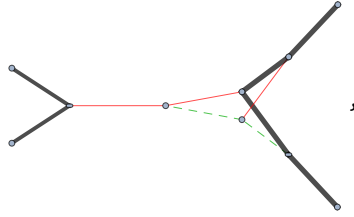

$$G^3 m_1^2 \left\{ \frac{-2 \hat{n} \times \vec{S}_1 \cdot \vec{v}_1 \hat{n} \times \vec{S}_2 \cdot \vec{v}_2 - \frac{2}{5} \vec{S}_1 \cdot \vec{v}_2 \vec{S}_2 \cdot \vec{v}_1 + \frac{2}{5} \vec{S}_1 \cdot \vec{S}_2 \vec{v}_1 \cdot \vec{v}_2}{r^5} \right\}$$

{DiagS1S2 [3, 1, 55],

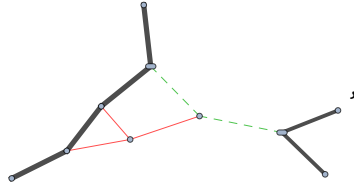

$$G^3 m_1^2 \left\{ \frac{1}{r^4} \left( 4 \hat{n} \cdot \vec{S}_2 \hat{n} \cdot \vec{S}_1 \hat{n} \cdot \vec{v}_1 + 4 \hat{n} \cdot \vec{S}_1 \hat{n} \cdot \vec{S}_2 \hat{n} \cdot \vec{v}_1 - \frac{92}{25} \vec{S}_1 \cdot \vec{S}_2 \hat{n} \cdot \vec{v}_1 - \frac{92}{25} \vec{S}_1 \cdot \vec{S}_2 \hat{n} \cdot \vec{v}_1 - \frac{32}{25} \hat{n} \cdot \vec{S}_2 \vec{S}_1 \cdot \vec{v}_1 + \frac{88}{25} \hat{n} \cdot \vec{S}_1 \vec{S}_2 \cdot \vec{v}_1 - \frac{32}{25} \hat{n} \cdot \vec{S}_2 \vec{S}_1 \cdot \vec{v}_1 + \frac{88}{25} \hat{n} \cdot \vec{S}_1 \vec{S}_2 \cdot \vec{v}_1 \right) + \frac{1}{r^5} \right. \\ \left( -29 \hat{n} \cdot \vec{S}_1 \hat{n} \cdot \vec{S}_2 (\hat{n} \cdot \vec{v}_1)^2 + 5 \vec{S}_1 \cdot \vec{S}_2 (\hat{n} \cdot \vec{v}_1)^2 + 16 \hat{n} \cdot \vec{S}_1 \hat{n} \cdot \vec{S}_2 \hat{n} \cdot \vec{v}_2 \hat{n} \cdot \vec{v}_1 - 16 \hat{n} \cdot \vec{v}_2 \vec{S}_1 \cdot \vec{S}_2 \hat{n} \cdot \vec{v}_1 + \right. \\ \left. 10 \hat{n} \cdot \vec{S}_2 \vec{S}_1 \cdot \vec{v}_1 \hat{n} \cdot \vec{v}_1 - 4 \hat{n} \cdot \vec{S}_2 \vec{S}_1 \cdot \vec{v}_2 \hat{n} \cdot \vec{v}_1 + 4 \hat{n} \cdot \vec{S}_1 \vec{S}_2 \cdot \vec{v}_1 \hat{n} \cdot \vec{v}_1 - 4 \hat{n} \cdot \vec{S}_1 \vec{S}_2 \cdot \vec{v}_2 \hat{n} \cdot \vec{v}_1 - \right. \\ \left. 6 \hat{n} \times \vec{S}_1 \cdot \vec{v}_1 \hat{n} \times \vec{S}_2 \cdot \vec{v}_1 - 4 \hat{n} \cdot \vec{S}_2 \hat{n} \cdot \vec{v}_2 \vec{S}_1 \cdot \vec{v}_1 + 20 \hat{n} \cdot \vec{S}_1 \hat{n} \cdot \vec{v}_2 \vec{S}_2 \cdot \vec{v}_1 - \frac{62}{25} \vec{S}_1 \cdot \vec{v}_1 \vec{S}_2 \cdot \vec{v}_1 - \frac{88}{25} \vec{S}_1 \cdot \vec{v}_2 \vec{S}_2 \cdot \vec{v}_1 + \right. \\ \left. \frac{32}{25} \vec{S}_1 \cdot \vec{v}_1 \vec{S}_2 \cdot \vec{v}_2 - 3 \hat{n} \cdot \vec{S}_1 \hat{n} \cdot \vec{S}_2 \vec{v}_1 \cdot \vec{v}_1 + \frac{119}{25} \vec{S}_1 \cdot \vec{S}_2 \vec{v}_1 \cdot \vec{v}_1 - 4 \hat{n} \cdot \vec{S}_1 \hat{n} \cdot \vec{S}_2 \vec{v}_1 \cdot \vec{v}_2 + \frac{92}{25} \vec{S}_1 \cdot \vec{S}_2 \vec{v}_1 \cdot \vec{v}_2 \right) + \\ \left. \frac{1}{r^4} \left( 12 \hat{n} \cdot \vec{S}_2 \hat{n} \cdot \vec{S}_1 \hat{n} \cdot \vec{v}_1 + 12 \hat{n} \cdot \vec{S}_1 \hat{n} \cdot \vec{S}_2 \hat{n} \cdot \vec{v}_1 - \frac{12}{5} \vec{S}_1 \cdot \vec{S}_2 \hat{n} \cdot \vec{v}_1 - \frac{12}{5} \vec{S}_1 \cdot \vec{S}_2 \hat{n} \cdot \vec{v}_1 - \right. \right. \\ \left. \frac{12}{5} \hat{n} \cdot \vec{S}_2 \vec{S}_1 \cdot \vec{v}_1 - \frac{12}{5} \hat{n} \cdot \vec{S}_1 \vec{S}_2 \cdot \vec{v}_1 - \frac{12}{5} \hat{n} \cdot \vec{S}_2 \vec{S}_1 \cdot \vec{v}_1 - \frac{12}{5} \hat{n} \cdot \vec{S}_1 \vec{S}_2 \cdot \vec{v}_1 \right) + \frac{1}{r^5} \\ \left( -42 \hat{n} \cdot \vec{S}_1 \hat{n} \cdot \vec{S}_2 (\hat{n} \cdot \vec{v}_1)^2 + 6 \vec{S}_1 \cdot \vec{S}_2 (\hat{n} \cdot \vec{v}_1)^2 + 84 \hat{n} \cdot \vec{S}_1 \hat{n} \cdot \vec{S}_2 \hat{n} \cdot \vec{v}_2 \hat{n} \cdot \vec{v}_1 - 12 \hat{n} \cdot \vec{v}_2 \vec{S}_1 \cdot \vec{S}_2 \hat{n} \cdot \vec{v}_1 + \right. \\ \left. 12 \hat{n} \cdot \vec{S}_2 \vec{S}_1 \cdot \vec{v}_1 \hat{n} \cdot \vec{v}_1 - 12 \hat{n} \cdot \vec{S}_2 \vec{S}_1 \cdot \vec{v}_2 \hat{n} \cdot \vec{v}_1 + 12 \hat{n} \cdot \vec{S}_1 \vec{S}_2 \cdot \vec{v}_1 \hat{n} \cdot \vec{v}_1 - 12 \hat{n} \cdot \vec{S}_1 \vec{S}_2 \cdot \vec{v}_2 \hat{n} \cdot \vec{v}_1 - \right. \\ \left. 12 \hat{n} \cdot \vec{S}_2 \hat{n} \cdot \vec{v}_2 \vec{S}_1 \cdot \vec{v}_1 - 12 \hat{n} \cdot \vec{S}_1 \hat{n} \cdot \vec{v}_2 \vec{S}_2 \cdot \vec{v}_1 - \frac{12}{5} \vec{S}_1 \cdot \vec{v}_1 \vec{S}_2 \cdot \vec{v}_1 + \frac{12}{5} \vec{S}_1 \cdot \vec{v}_2 \vec{S}_2 \cdot \vec{v}_1 + \frac{12}{5} \vec{S}_1 \cdot \vec{v}_1 \vec{S}_2 \cdot \vec{v}_2 + \right. \\ \left. 6 \hat{n} \cdot \vec{S}_1 \hat{n} \cdot \vec{S}_2 \vec{v}_1 \cdot \vec{v}_1 - \frac{6}{5} \vec{S}_1 \cdot \vec{S}_2 \vec{v}_1 \cdot \vec{v}_1 - 12 \hat{n} \cdot \vec{S}_1 \hat{n} \cdot \vec{S}_2 \vec{v}_1 \cdot \vec{v}_2 + \frac{12}{5} \vec{S}_1 \cdot \vec{S}_2 \vec{v}_1 \cdot \vec{v}_2 \right) \log \left( \frac{r}{R_0} \right) +$$

$$\frac{1}{\epsilon_d} \left( \frac{1}{r^4} \left( -4 \hat{n} \cdot \vec{S}_2 \hat{n} \cdot \vec{S}_1 \hat{n} \cdot \vec{v}_1 - 4 \hat{n} \cdot \vec{S}_1 \hat{n} \cdot \vec{S}_2 \hat{n} \cdot \vec{v}_1 + \frac{4}{5} \vec{S}_1 \cdot \vec{S}_2 \hat{n} \cdot \vec{v}_1 + \frac{4}{5} \vec{S}_1 \cdot \vec{S}_2 \hat{n} \cdot \vec{v}_1 + \right. \right. \\ \left. \left. \frac{4}{5} \hat{n} \cdot \vec{S}_2 \vec{S}_1 \cdot \vec{v}_1 + \frac{4}{5} \hat{n} \cdot \vec{S}_1 \vec{S}_2 \cdot \vec{v}_1 + \frac{4}{5} \hat{n} \cdot \vec{S}_2 \vec{S}_1 \cdot \vec{v}_1 + \frac{4}{5} \hat{n} \cdot \vec{S}_1 \vec{S}_2 \cdot \vec{v}_1 \right) + \frac{1}{r^5} \right. \\ \left. \left( 14 \hat{n} \cdot \vec{S}_1 \hat{n} \cdot \vec{S}_2 (\hat{n} \cdot \vec{v}_1)^2 - 2 \vec{S}_1 \cdot \vec{S}_2 (\hat{n} \cdot \vec{v}_1)^2 - 28 \hat{n} \cdot \vec{S}_1 \hat{n} \cdot \vec{S}_2 \hat{n} \cdot \vec{v}_2 \hat{n} \cdot \vec{v}_1 + 4 \hat{n} \cdot \vec{v}_2 \vec{S}_1 \cdot \vec{S}_2 \hat{n} \cdot \vec{v}_1 - \right. \right. \\ \left. \left. 4 \hat{n} \cdot \vec{S}_2 \vec{S}_1 \cdot \vec{v}_1 \hat{n} \cdot \vec{v}_1 + 4 \hat{n} \cdot \vec{S}_2 \vec{S}_1 \cdot \vec{v}_2 \hat{n} \cdot \vec{v}_1 - 4 \hat{n} \cdot \vec{S}_1 \vec{S}_2 \cdot \vec{v}_1 \hat{n} \cdot \vec{v}_1 + 4 \hat{n} \cdot \vec{S}_1 \vec{S}_2 \cdot \vec{v}_2 \hat{n} \cdot \vec{v}_1 + \right. \right. \\ \left. \left. 4 \hat{n} \cdot \vec{S}_2 \hat{n} \cdot \vec{v}_2 \vec{S}_1 \cdot \vec{v}_1 + 4 \hat{n} \cdot \vec{S}_1 \hat{n} \cdot \vec{v}_2 \vec{S}_2 \cdot \vec{v}_1 + \frac{4}{5} \vec{S}_1 \cdot \vec{v}_1 \vec{S}_2 \cdot \vec{v}_1 - \frac{4}{5} \vec{S}_1 \cdot \vec{v}_2 \vec{S}_2 \cdot \vec{v}_1 - \frac{4}{5} \vec{S}_1 \cdot \vec{v}_1 \vec{S}_2 \cdot \vec{v}_2 - \right. \right. \\ \left. \left. 2 \hat{n} \cdot \vec{S}_1 \hat{n} \cdot \vec{S}_2 \vec{v}_1 \cdot \vec{v}_1 + \frac{2}{5} \vec{S}_1 \cdot \vec{S}_2 \vec{v}_1 \cdot \vec{v}_1 + 4 \hat{n} \cdot \vec{S}_1 \hat{n} \cdot \vec{S}_2 \vec{v}_1 \cdot \vec{v}_2 - \frac{4}{5} \vec{S}_1 \cdot \vec{S}_2 \vec{v}_1 \cdot \vec{v}_2 \right) \right) \Bigg\}$$

{DiagS1S2 [3, 1, 56],

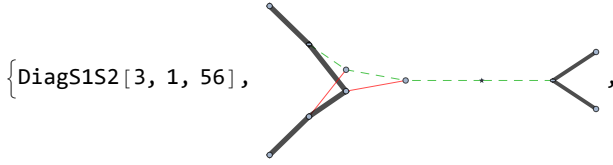

$$G^3 m_1^2 \left( \frac{\frac{47}{25} \hat{n} \cdot \vec{S}_1 \hat{n} \cdot \vec{S}_2 - \frac{107}{75} \vec{S}_1 \cdot \vec{S}_2}{r^3} + \frac{1}{r^4} \left( -13 \hat{n} \cdot \vec{S}_2 \hat{n} \cdot \vec{S}_1 \hat{n} \cdot \vec{v}_1 + \frac{137}{25} \vec{S}_1 \cdot \vec{S}_2 \hat{n} \cdot \vec{v}_1 + 13 \hat{n} \cdot \vec{S}_1 \hat{n} \cdot \vec{S}_2 \hat{n} \cdot \vec{v}_2 - \right. \right. \\ \left. \left. \frac{137}{25} \hat{n} \cdot \vec{v}_2 \vec{S}_1 \cdot \vec{S}_2 - \frac{47}{25} \hat{n} \cdot \vec{S}_2 \vec{S}_1 \cdot \vec{v}_2 + \frac{47}{25} \hat{n} \cdot \vec{S}_1 \vec{S}_2 \cdot \vec{v}_1 + \frac{47}{25} \hat{n} \cdot \vec{S}_2 \vec{S}_1 \cdot \vec{v}_1 - \frac{47}{25} \hat{n} \cdot \vec{S}_1 \vec{S}_2 \cdot \vec{v}_2 \right) + \right. \\ \left. \frac{1}{r^5} \left( -109 \hat{n} \cdot \vec{S}_1 \hat{n} \cdot \vec{S}_2 \hat{n} \cdot \vec{v}_1 \hat{n} \cdot \vec{v}_2 + 31 \hat{n} \cdot \vec{v}_1 \vec{S}_1 \cdot \vec{S}_2 \hat{n} \cdot \vec{v}_2 + 13 \hat{n} \cdot \vec{S}_2 \vec{S}_1 \cdot \vec{v}_1 \hat{n} \cdot \vec{v}_2 + \right. \right. \\ \left. \left. 13 \hat{n} \cdot \vec{S}_1 \vec{S}_2 \cdot \vec{v}_1 \hat{n} \cdot \vec{v}_2 + 13 \hat{n} \cdot \vec{S}_2 \hat{n} \cdot \vec{v}_1 \vec{S}_1 \cdot \vec{v}_2 - \frac{47}{25} \vec{S}_1 \cdot \vec{v}_2 \vec{S}_2 \cdot \vec{v}_1 + \right. \right. \\ \left. \left. 13 \hat{n} \cdot \vec{S}_1 \hat{n} \cdot \vec{v}_1 \vec{S}_2 \cdot \vec{v}_2 - \frac{47}{25} \vec{S}_1 \cdot \vec{v}_1 \vec{S}_2 \cdot \vec{v}_2 + 13 \hat{n} \cdot \vec{S}_1 \hat{n} \cdot \vec{S}_2 \vec{v}_1 \cdot \vec{v}_2 - \frac{137}{25} \vec{S}_1 \cdot \vec{S}_2 \vec{v}_1 \cdot \vec{v}_2 \right) + \right. \\ \left. \left( \frac{\frac{6}{5} \vec{S}_1 \cdot \vec{S}_2 - \frac{18}{5} \hat{n} \cdot \vec{S}_1 \hat{n} \cdot \vec{S}_2}{r^3} + \frac{1}{r^4} \left( 18 \hat{n} \cdot \vec{S}_2 \hat{n} \cdot \vec{S}_1 \hat{n} \cdot \vec{v}_1 - \frac{18}{5} \vec{S}_1 \cdot \vec{S}_2 \hat{n} \cdot \vec{v}_1 - 18 \hat{n} \cdot \vec{S}_1 \hat{n} \cdot \vec{S}_2 \hat{n} \cdot \vec{v}_2 + \frac{18}{5} \hat{n} \cdot \vec{v}_2 \vec{S}_1 \cdot \vec{S}_2 + \right. \right. \\ \left. \left. \frac{18}{5} \hat{n} \cdot \vec{S}_2 \vec{S}_1 \cdot \vec{v}_2 - \frac{18}{5} \hat{n} \cdot \vec{S}_1 \vec{S}_2 \cdot \vec{v}_1 - \frac{18}{5} \hat{n} \cdot \vec{S}_2 \vec{S}_1 \cdot \vec{v}_1 + \frac{18}{5} \hat{n} \cdot \vec{S}_1 \vec{S}_2 \cdot \vec{v}_2 \right) + \frac{1}{r^5} \left( 126 \hat{n} \cdot \vec{S}_1 \hat{n} \cdot \vec{S}_2 \hat{n} \cdot \vec{v}_1 \hat{n} \cdot \vec{v}_2 - \right. \right. \\ \left. \left. 18 \hat{n} \cdot \vec{v}_1 \vec{S}_1 \cdot \vec{S}_2 \hat{n} \cdot \vec{v}_2 - 18 \hat{n} \cdot \vec{S}_2 \vec{S}_1 \cdot \vec{v}_1 \hat{n} \cdot \vec{v}_2 - 18 \hat{n} \cdot \vec{S}_1 \vec{S}_2 \cdot \vec{v}_1 \hat{n} \cdot \vec{v}_2 - 18 \hat{n} \cdot \vec{S}_2 \hat{n} \cdot \vec{v}_1 \vec{S}_1 \cdot \vec{v}_2 + \frac{18}{5} \vec{S}_1 \cdot \vec{v}_2 \right. \right. \\ \left. \left. \vec{S}_2 \cdot \vec{v}_1 - 18 \hat{n} \cdot \vec{S}_1 \hat{n} \cdot \vec{v}_1 \vec{S}_2 \cdot \vec{v}_2 + \frac{18}{5} \vec{S}_1 \cdot \vec{v}_1 \vec{S}_2 \cdot \vec{v}_2 - 18 \hat{n} \cdot \vec{S}_1 \hat{n} \cdot \vec{S}_2 \vec{v}_1 \cdot \vec{v}_2 + \frac{18}{5} \vec{S}_1 \cdot \vec{S}_2 \vec{v}_1 \cdot \vec{v}_2 \right) \right) \log \left( \frac{r}{R_0} \right) + \\ \frac{1}{\epsilon_d} \left( \frac{\frac{6}{5} \hat{n} \cdot \vec{S}_1 \hat{n} \cdot \vec{S}_2 - \frac{2}{5} \vec{S}_1 \cdot \vec{S}_2}{r^3} + \frac{1}{r^4} \left( -6 \hat{n} \cdot \vec{S}_2 \hat{n} \cdot \vec{S}_1 \hat{n} \cdot \vec{v}_1 + \frac{6}{5} \vec{S}_1 \cdot \vec{S}_2 \hat{n} \cdot \vec{v}_1 + 6 \hat{n} \cdot \vec{S}_1 \hat{n} \cdot \vec{S}_2 \hat{n} \cdot \vec{v}_2 - \right. \right. \\ \left. \left. \frac{6}{5} \hat{n} \cdot \vec{v}_2 \vec{S}_1 \cdot \vec{S}_2 - \frac{6}{5} \hat{n} \cdot \vec{S}_2 \vec{S}_1 \cdot \vec{v}_2 + \frac{6}{5} \hat{n} \cdot \vec{S}_1 \vec{S}_2 \cdot \vec{v}_1 + \frac{6}{5} \hat{n} \cdot \vec{S}_2 \vec{S}_1 \cdot \vec{v}_1 - \frac{6}{5} \hat{n} \cdot \vec{S}_1 \vec{S}_2 \cdot \vec{v}_2 \right) + \frac{1}{r^5} \right. \\ \left. \left( -42 \hat{n} \cdot \vec{S}_1 \hat{n} \cdot \vec{S}_2 \hat{n} \cdot \vec{v}_1 \hat{n} \cdot \vec{v}_2 + 6 \hat{n} \cdot \vec{v}_1 \vec{S}_1 \cdot \vec{S}_2 \hat{n} \cdot \vec{v}_2 + 6 \hat{n} \cdot \vec{S}_2 \vec{S}_1 \cdot \vec{v}_1 \hat{n} \cdot \vec{v}_2 + 6 \hat{n} \cdot \vec{S}_1 \vec{S}_2 \cdot \vec{v}_1 \hat{n} \cdot \vec{v}_2 + 6 \hat{n} \cdot \vec{S}_2 \hat{n} \cdot \vec{v}_1 \right. \right. \\ \left. \left. \vec{S}_1 \cdot \vec{v}_2 - \frac{6}{5} \vec{S}_1 \cdot \vec{v}_2 \vec{S}_2 \cdot \vec{v}_1 + 6 \hat{n} \cdot \vec{S}_1 \hat{n} \cdot \vec{v}_1 \vec{S}_2 \cdot \vec{v}_2 - \frac{6}{5} \vec{S}_1 \cdot \vec{v}_1 \vec{S}_2 \cdot \vec{v}_2 + 6 \hat{n} \cdot \vec{S}_1 \hat{n} \cdot \vec{S}_2 \vec{v}_1 \cdot \vec{v}_2 - \frac{6}{5} \vec{S}_1 \cdot \vec{S}_2 \vec{v}_1 \cdot \vec{v}_2 \right) \right) \Bigg\}$$

{DiagS1S2[3, 1, 57],

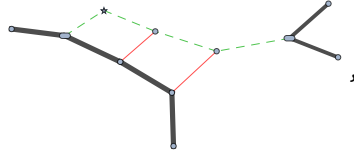

$$\begin{aligned}
 G^3 m_1^2 & \left( \frac{-4 \hat{n} \cdot \vec{S}_1 \hat{n} \cdot \vec{S}_2 - \frac{20}{3} \vec{S}_1 \cdot \vec{S}_2}{r^3} + \frac{1}{r^4} \left( -16 \hat{n} \cdot \vec{S}_1 \hat{n} \cdot \vec{S}_2 \hat{n} \cdot \vec{v}_1 + \frac{474}{25} \vec{S}_1 \cdot \vec{S}_2 \hat{n} \cdot \vec{v}_1 + \frac{326}{25} \vec{S}_1 \cdot \vec{S}_2 \hat{n} \cdot \vec{v}_1 + \right. \right. \\
 & 16 \hat{n} \cdot \vec{S}_1 \hat{n} \cdot \vec{S}_2 \hat{n} \cdot \vec{v}_2 - 32 \hat{n} \cdot \vec{v}_2 \vec{S}_1 \cdot \vec{S}_2 - \frac{46}{25} \hat{n} \cdot \vec{S}_2 \vec{S}_1 \cdot \vec{v}_1 + 4 \hat{n} \cdot \vec{S}_2 \vec{S}_1 \cdot \vec{v}_2 - \frac{164}{25} \hat{n} \cdot \vec{S}_1 \vec{S}_2 \cdot \vec{v}_1 - \\
 & \frac{54}{25} \hat{n} \cdot \vec{S}_2 \vec{S}_1 \cdot \vec{v}_1 + \frac{64}{25} \hat{n} \cdot \vec{S}_1 \vec{S}_2 \cdot \vec{v}_1 + 4 \hat{n} \cdot \vec{S}_1 \vec{S}_2 \cdot \vec{v}_2 \Big) + \frac{1}{r^5} \left( 54 \hat{n} \cdot \vec{S}_1 \hat{n} \cdot \vec{S}_2 (\hat{n} \cdot \vec{v}_1)^2 - \frac{2064}{49} \vec{S}_1 \cdot \vec{S}_2 (\hat{n} \cdot \vec{v}_1)^2 - \right. \\
 & 54 \hat{n} \cdot \vec{S}_1 \hat{n} \cdot \vec{S}_2 \hat{n} \cdot \vec{v}_2 \hat{n} \cdot \vec{v}_1 + 76 \hat{n} \cdot \vec{v}_2 \vec{S}_1 \cdot \vec{S}_2 \hat{n} \cdot \vec{v}_1 - \frac{432}{49} \hat{n} \cdot \vec{S}_2 \vec{S}_1 \cdot \vec{v}_1 \hat{n} \cdot \vec{v}_1 + \frac{282}{49} \hat{n} \cdot \vec{S}_1 \vec{S}_2 \cdot \vec{v}_1 \hat{n} \cdot \vec{v}_1 - \\
 & \frac{76}{7} \hat{n} \times \vec{S}_1 \cdot \vec{v}_1 \hat{n} \times \vec{S}_2 \cdot \vec{v}_1 - 22 \hat{n} \cdot \vec{S}_1 \hat{n} \cdot \vec{v}_2 \vec{S}_2 \cdot \vec{v}_1 - \frac{6338 \vec{S}_1 \cdot \vec{v}_1 \vec{S}_2 \cdot \vec{v}_1}{1225} + \frac{164}{25} \vec{S}_1 \cdot \vec{v}_2 \vec{S}_2 \cdot \vec{v}_1 + \\
 & \left. \frac{54}{25} \vec{S}_1 \cdot \vec{v}_1 \vec{S}_2 \cdot \vec{v}_2 - \frac{132}{49} \hat{n} \cdot \vec{S}_1 \hat{n} \cdot \vec{S}_2 \vec{v}_1 \cdot \vec{v}_1 + \frac{10586 \vec{S}_1 \cdot \vec{S}_2 \vec{v}_1 \cdot \vec{v}_1}{1225} - \frac{326}{25} \vec{S}_1 \cdot \vec{S}_2 \vec{v}_1 \cdot \vec{v}_2 \right) + \\
 & \left( \frac{12 \vec{S}_1 \cdot \vec{S}_2 - 36 \hat{n} \cdot \vec{S}_1 \hat{n} \cdot \vec{S}_2}{r^3} + \frac{1}{r^4} \left( 54 \hat{n} \cdot \vec{S}_2 \hat{n} \cdot \vec{S}_1 \hat{n} \cdot \vec{v}_1 + 126 \hat{n} \cdot \vec{S}_1 \hat{n} \cdot \vec{S}_2 \hat{n} \cdot \vec{v}_1 - \frac{126}{5} \vec{S}_1 \cdot \vec{S}_2 \hat{n} \cdot \vec{v}_1 - \right. \right. \\
 & \frac{54}{5} \vec{S}_1 \cdot \vec{S}_2 \hat{n} \cdot \vec{v}_1 - 180 \hat{n} \cdot \vec{S}_1 \hat{n} \cdot \vec{S}_2 \hat{n} \cdot \vec{v}_2 + 36 \hat{n} \cdot \vec{v}_2 \vec{S}_1 \cdot \vec{S}_2 - \frac{126}{5} \hat{n} \cdot \vec{S}_2 \vec{S}_1 \cdot \vec{v}_1 + \\
 & 36 \hat{n} \cdot \vec{S}_2 \vec{S}_1 \cdot \vec{v}_2 - \frac{54}{5} \hat{n} \cdot \vec{S}_1 \vec{S}_2 \cdot \vec{v}_1 - \frac{54}{5} \hat{n} \cdot \vec{S}_2 \vec{S}_1 \cdot \vec{v}_1 - \frac{126}{5} \hat{n} \cdot \vec{S}_1 \vec{S}_2 \cdot \vec{v}_1 + 36 \hat{n} \cdot \vec{S}_1 \vec{S}_2 \cdot \vec{v}_2 \Big) + \frac{1}{r^5} \\
 & \left( -162 \hat{n} \cdot \vec{S}_1 \hat{n} \cdot \vec{S}_2 (\hat{n} \cdot \vec{v}_1)^2 + \frac{162}{7} \vec{S}_1 \cdot \vec{S}_2 (\hat{n} \cdot \vec{v}_1)^2 + 378 \hat{n} \cdot \vec{S}_1 \hat{n} \cdot \vec{S}_2 \hat{n} \cdot \vec{v}_2 \hat{n} \cdot \vec{v}_1 - 54 \hat{n} \cdot \vec{v}_2 \vec{S}_1 \cdot \vec{S}_2 \hat{n} \cdot \vec{v}_1 + \right. \\
 & \frac{324}{7} \hat{n} \cdot \vec{S}_2 \vec{S}_1 \cdot \vec{v}_1 \hat{n} \cdot \vec{v}_1 - 54 \hat{n} \cdot \vec{S}_2 \vec{S}_1 \cdot \vec{v}_2 \hat{n} \cdot \vec{v}_1 + \frac{324}{7} \hat{n} \cdot \vec{S}_1 \vec{S}_2 \cdot \vec{v}_1 \hat{n} \cdot \vec{v}_1 - 54 \hat{n} \cdot \vec{S}_1 \vec{S}_2 \cdot \vec{v}_2 \hat{n} \cdot \vec{v}_1 - \\
 & 54 \hat{n} \cdot \vec{S}_2 \hat{n} \cdot \vec{v}_2 \vec{S}_1 \cdot \vec{v}_1 - 54 \hat{n} \cdot \vec{S}_1 \hat{n} \cdot \vec{v}_2 \vec{S}_2 \cdot \vec{v}_1 - \frac{324}{35} \vec{S}_1 \cdot \vec{v}_1 \vec{S}_2 \cdot \vec{v}_1 + \frac{54}{5} \vec{S}_1 \cdot \vec{v}_2 \vec{S}_2 \cdot \vec{v}_1 + \frac{54}{5} \vec{S}_1 \cdot \vec{v}_1 \vec{S}_2 \cdot \vec{v}_2 + \\
 & \left. \frac{162}{7} \hat{n} \cdot \vec{S}_1 \hat{n} \cdot \vec{S}_2 \vec{v}_1 \cdot \vec{v}_1 - \frac{162}{35} \vec{S}_1 \cdot \vec{S}_2 \vec{v}_1 \cdot \vec{v}_1 - 54 \hat{n} \cdot \vec{S}_1 \hat{n} \cdot \vec{S}_2 \vec{v}_1 \cdot \vec{v}_2 + \frac{54}{5} \vec{S}_1 \cdot \vec{S}_2 \vec{v}_1 \cdot \vec{v}_2 \right) \log \left( \frac{r}{R_\theta} \right) + \\
 & \frac{1}{\epsilon_d} \left( \frac{12 \hat{n} \cdot \vec{S}_1 \hat{n} \cdot \vec{S}_2 - 4 \vec{S}_1 \cdot \vec{S}_2}{r^3} + \frac{1}{r^4} \left( -18 \hat{n} \cdot \vec{S}_2 \hat{n} \cdot \vec{S}_1 \hat{n} \cdot \vec{v}_1 - 42 \hat{n} \cdot \vec{S}_1 \hat{n} \cdot \vec{S}_2 \hat{n} \cdot \vec{v}_1 + \frac{42}{5} \vec{S}_1 \cdot \vec{S}_2 \hat{n} \cdot \vec{v}_1 + \right. \right. \\
 & \frac{18}{5} \vec{S}_1 \cdot \vec{S}_2 \hat{n} \cdot \vec{v}_1 + 60 \hat{n} \cdot \vec{S}_1 \hat{n} \cdot \vec{S}_2 \hat{n} \cdot \vec{v}_2 - 12 \hat{n} \cdot \vec{v}_2 \vec{S}_1 \cdot \vec{S}_2 + \frac{42}{5} \hat{n} \cdot \vec{S}_2 \vec{S}_1 \cdot \vec{v}_1 - \\
 & 12 \hat{n} \cdot \vec{S}_2 \vec{S}_1 \cdot \vec{v}_2 + \frac{18}{5} \hat{n} \cdot \vec{S}_1 \vec{S}_2 \cdot \vec{v}_1 + \frac{18}{5} \hat{n} \cdot \vec{S}_2 \vec{S}_1 \cdot \vec{v}_1 + \frac{42}{5} \hat{n} \cdot \vec{S}_1 \vec{S}_2 \cdot \vec{v}_1 - 12 \hat{n} \cdot \vec{S}_1 \vec{S}_2 \cdot \vec{v}_2 \Big) + \frac{1}{r^5} \\
 & \left( 54 \hat{n} \cdot \vec{S}_1 \hat{n} \cdot \vec{S}_2 (\hat{n} \cdot \vec{v}_1)^2 - \frac{54}{7} \vec{S}_1 \cdot \vec{S}_2 (\hat{n} \cdot \vec{v}_1)^2 - 126 \hat{n} \cdot \vec{S}_1 \hat{n} \cdot \vec{S}_2 \hat{n} \cdot \vec{v}_2 \hat{n} \cdot \vec{v}_1 + 18 \hat{n} \cdot \vec{v}_2 \vec{S}_1 \cdot \vec{S}_2 \hat{n} \cdot \vec{v}_1 - \right. \\
 & \frac{108}{7} \hat{n} \cdot \vec{S}_2 \vec{S}_1 \cdot \vec{v}_1 \hat{n} \cdot \vec{v}_1 + 18 \hat{n} \cdot \vec{S}_2 \vec{S}_1 \cdot \vec{v}_2 \hat{n} \cdot \vec{v}_1 - \frac{108}{7} \hat{n} \cdot \vec{S}_1 \vec{S}_2 \cdot \vec{v}_1 \hat{n} \cdot \vec{v}_1 + 18 \hat{n} \cdot \vec{S}_1 \vec{S}_2 \cdot \vec{v}_2 \hat{n} \cdot \vec{v}_1 + \\
 & 18 \hat{n} \cdot \vec{S}_2 \hat{n} \cdot \vec{v}_2 \vec{S}_1 \cdot \vec{v}_1 + 18 \hat{n} \cdot \vec{S}_1 \hat{n} \cdot \vec{v}_2 \vec{S}_2 \cdot \vec{v}_1 + \frac{108}{35} \vec{S}_1 \cdot \vec{v}_1 \vec{S}_2 \cdot \vec{v}_1 - \frac{18}{5} \vec{S}_1 \cdot \vec{v}_2 \vec{S}_2 \cdot \vec{v}_1 - \frac{18}{5} \vec{S}_1 \cdot \vec{v}_1 \vec{S}_2 \cdot \vec{v}_2 -
 \end{aligned}$$

$$\left. \left. \left. \frac{54}{7} \hat{n} \cdot \vec{S}_1 \hat{n} \cdot \vec{S}_2 \vec{v}_1 \cdot \vec{v}_1 + \frac{54}{35} \vec{S}_1 \cdot \vec{S}_2 \vec{v}_1 \cdot \vec{v}_1 + 18 \hat{n} \cdot \vec{S}_1 \hat{n} \cdot \vec{S}_2 \vec{v}_1 \cdot \vec{v}_2 - \frac{18}{5} \vec{S}_1 \cdot \vec{S}_2 \vec{v}_1 \cdot \vec{v}_2 \right) \right) \right\}$$

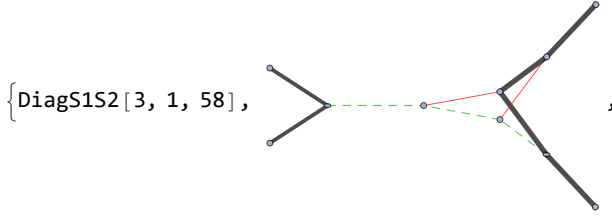

$$G^3 m_1^2 \left( \frac{1}{r^4} \left( \frac{24}{5} \vec{S}_1 \cdot \vec{a}_2 \hat{n} \cdot \vec{S}_2 + 32 \vec{S}_1 \cdot \vec{S}_2 \hat{n} \cdot \vec{a}_1 - \frac{24}{5} \vec{S}_1 \cdot \vec{S}_2 \hat{n} \cdot \vec{a}_2 - 32 \vec{S}_2 \cdot \vec{a}_1 \hat{n} \cdot \vec{S}_1 + 32 \vec{S}_1 \cdot \vec{S}_2 \hat{n} \cdot \vec{v}_1 - \frac{24}{5} \vec{S}_1 \cdot \vec{S}_2 \hat{n} \cdot \vec{v}_2 + \right. \right. \\ \left. \frac{24}{5} \hat{n} \cdot \vec{S}_2 \vec{S}_1 \cdot \vec{v}_2 - 32 \hat{n} \cdot \vec{S}_1 \vec{S}_2 \cdot \vec{v}_1 \right) + \frac{1}{r^5} \left( 54 \hat{n} \times \vec{S}_1 \cdot \vec{v}_1 \hat{n} \times \vec{S}_2 \cdot \vec{v}_1 + 18 \hat{n} \times \vec{S}_1 \cdot \vec{v}_2 \hat{n} \times \vec{S}_2 \cdot \vec{v}_2 - \right. \\ \left. 42 \vec{S}_1 \cdot \vec{S}_2 (\hat{n} \cdot \vec{v}_1)^2 + 42 \hat{n} \cdot \vec{S}_1 \hat{n} \cdot \vec{v}_1 \vec{S}_2 \cdot \vec{v}_1 - 6 \vec{S}_1 \cdot \vec{S}_2 (\hat{n} \cdot \vec{v}_2)^2 + 6 \hat{n} \cdot \vec{S}_2 \hat{n} \cdot \vec{v}_2 \vec{S}_1 \cdot \vec{v}_2 - \right. \\ \left. 36 \vec{v}_1 \cdot \vec{v}_1 \hat{n} \cdot \vec{S}_1 \hat{n} \cdot \vec{S}_2 + \frac{12}{5} \vec{S}_1 \cdot \vec{v}_1 \vec{S}_2 \cdot \vec{v}_1 + \frac{12}{5} \vec{S}_1 \cdot \vec{v}_2 \vec{S}_2 \cdot \vec{v}_2 + \frac{96}{5} \vec{S}_1 \cdot \vec{S}_2 \vec{v}_1 \cdot \vec{v}_1 - \frac{12}{5} \vec{S}_1 \cdot \vec{S}_2 \vec{v}_2 \cdot \vec{v}_2 \right) \Bigg\}$$

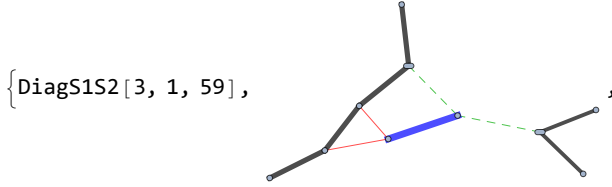

$$G^3 m_1^2 \left( \frac{\frac{1}{4} \hat{n} \cdot \vec{S}_1 \hat{n} \cdot \vec{S}_2 - \frac{1}{12} \vec{S}_1 \cdot \vec{S}_2}{r^3} + \frac{1}{r^4} \left( -\frac{3}{4} \hat{n} \cdot \vec{S}_2 \hat{n} \cdot \vec{S}_1 \hat{n} \cdot \vec{v}_1 + \frac{2}{5} \vec{S}_1 \cdot \vec{S}_2 \hat{n} \cdot \vec{v}_1 + \frac{1}{4} \vec{S}_1 \cdot \vec{S}_2 \hat{n} \cdot \vec{v}_1 + \frac{5}{4} \hat{n} \cdot \vec{S}_1 \hat{n} \cdot \vec{S}_2 \hat{n} \cdot \vec{v}_2 - \right. \right. \\ \left. \frac{1}{4} \hat{n} \cdot \vec{v}_2 \vec{S}_1 \cdot \vec{S}_2 - \frac{1}{4} \hat{n} \cdot \vec{S}_2 \vec{S}_1 \cdot \vec{v}_2 + \frac{1}{20} \hat{n} \cdot \vec{S}_1 \vec{S}_2 \cdot \vec{v}_1 - \frac{2}{5} \hat{n} \cdot \vec{v}_2 \vec{S}_1 \cdot \vec{S}_2 + \frac{2}{5} \hat{n} \cdot \vec{S}_2 \vec{S}_1 \cdot \vec{a}_2 + \frac{2}{5} \hat{n} \cdot \vec{a}_1 \vec{S}_1 \cdot \vec{S}_2 - \right. \\ \left. \frac{2}{5} \hat{n} \cdot \vec{a}_2 \vec{S}_1 \cdot \vec{S}_2 + \frac{3}{20} \hat{n} \cdot \vec{S}_2 \vec{S}_1 \cdot \vec{v}_1 + \frac{2}{5} \hat{n} \cdot \vec{S}_2 \vec{S}_1 \cdot \vec{v}_2 - \frac{2}{5} \hat{n} \cdot \vec{S}_1 \vec{S}_2 \cdot \vec{a}_1 - \frac{2}{5} \hat{n} \cdot \vec{S}_1 \vec{S}_2 \cdot \vec{v}_1 - \frac{1}{4} \hat{n} \cdot \vec{S}_1 \vec{S}_2 \cdot \vec{v}_2 \right) + \\ \left. \frac{1}{r^5} \left( -\frac{61}{49} \vec{S}_1 \cdot \vec{S}_2 (\hat{n} \cdot \vec{v}_1)^2 - \frac{21}{4} \hat{n} \cdot \vec{S}_1 \hat{n} \cdot \vec{S}_2 \hat{n} \cdot \vec{v}_2 \hat{n} \cdot \vec{v}_1 + \frac{5}{4} \hat{n} \cdot \vec{v}_2 \vec{S}_1 \cdot \vec{S}_2 \hat{n} \cdot \vec{v}_1 - \frac{3}{49} \hat{n} \cdot \vec{S}_2 \vec{S}_1 \cdot \vec{v}_1 \hat{n} \cdot \vec{v}_1 + \right. \right. \\ \left. \frac{3}{4} \hat{n} \cdot \vec{S}_2 \vec{S}_1 \cdot \vec{v}_2 \hat{n} \cdot \vec{v}_1 + \frac{67}{49} \hat{n} \cdot \vec{S}_1 \vec{S}_2 \cdot \vec{v}_1 \hat{n} \cdot \vec{v}_1 + \frac{3}{4} \hat{n} \cdot \vec{S}_1 \vec{S}_2 \cdot \vec{v}_2 \hat{n} \cdot \vec{v}_1 + \frac{11}{7} \hat{n} \times \vec{S}_1 \cdot \vec{v}_1 \hat{n} \times \vec{S}_2 \cdot \vec{v}_1 + \right. \\ \left. \frac{3}{2} \hat{n} \times \vec{S}_1 \cdot \vec{v}_2 \hat{n} \times \vec{S}_2 \cdot \vec{v}_2 - \frac{1}{2} (\hat{n} \cdot \vec{v}_2)^2 \vec{S}_1 \cdot \vec{S}_2 + \frac{3}{4} \hat{n} \cdot \vec{S}_2 \hat{n} \cdot \vec{v}_2 \vec{S}_1 \cdot \vec{v}_1 + \frac{1}{2} \hat{n} \cdot \vec{S}_2 \hat{n} \cdot \vec{v}_2 \vec{S}_1 \cdot \vec{v}_2 + \right. \\ \left. \frac{1}{4} \hat{n} \cdot \vec{S}_1 \hat{n} \cdot \vec{v}_2 \vec{S}_2 \cdot \vec{v}_1 + \frac{71 \vec{S}_1 \cdot \vec{v}_1 \vec{S}_2 \cdot \vec{v}_1}{1225} - \frac{1}{20} \vec{S}_1 \cdot \vec{v}_2 \vec{S}_2 \cdot \vec{v}_1 - \frac{3}{20} \vec{S}_1 \cdot \vec{v}_1 \vec{S}_2 \cdot \vec{v}_2 + \frac{1}{5} \vec{S}_1 \cdot \vec{v}_2 \vec{S}_2 \cdot \vec{v}_2 - \right. \\ \left. \frac{353}{98} \hat{n} \cdot \vec{S}_1 \hat{n} \cdot \vec{S}_2 \vec{v}_1 \cdot \vec{v}_1 + \frac{5111 \vec{S}_1 \cdot \vec{S}_2 \vec{v}_1 \cdot \vec{v}_1}{2450} + \frac{3}{4} \hat{n} \cdot \vec{S}_1 \hat{n} \cdot \vec{S}_2 \vec{v}_1 \cdot \vec{v}_2 - \frac{1}{4} \vec{S}_1 \cdot \vec{S}_2 \vec{v}_1 \cdot \vec{v}_2 - \frac{1}{5} \vec{S}_1 \cdot \vec{S}_2 \vec{v}_2 \cdot \vec{v}_2 \right) + \\ \left. \frac{1}{r^5} \left( \frac{3}{2} \hat{n} \cdot \vec{S}_1 \hat{n} \cdot \vec{S}_2 (\hat{n} \cdot \vec{v}_1)^2 - \frac{3}{14} \vec{S}_1 \cdot \vec{S}_2 (\hat{n} \cdot \vec{v}_1)^2 - \frac{3}{7} \hat{n} \cdot \vec{S}_2 \vec{S}_1 \cdot \vec{v}_1 \hat{n} \cdot \vec{v}_1 - \frac{3}{7} \hat{n} \cdot \vec{S}_1 \vec{S}_2 \cdot \vec{v}_1 \hat{n} \cdot \vec{v}_1 + \right. \right. \\ \left. \frac{3}{35} \vec{S}_1 \cdot \vec{v}_1 \vec{S}_2 \cdot \vec{v}_1 - \frac{3}{14} \hat{n} \cdot \vec{S}_1 \hat{n} \cdot \vec{S}_2 \vec{v}_1 \cdot \vec{v}_1 + \frac{3}{70} \vec{S}_1 \cdot \vec{S}_2 \vec{v}_1 \cdot \vec{v}_1 \right) \log \left( \frac{r}{R_0} \right) + \frac{1}{r^5 \epsilon_d} \\ \left( -\frac{1}{2} \hat{n} \cdot \vec{S}_1 \hat{n} \cdot \vec{S}_2 (\hat{n} \cdot \vec{v}_1)^2 + \frac{1}{14} \vec{S}_1 \cdot \vec{S}_2 (\hat{n} \cdot \vec{v}_1)^2 + \frac{1}{7} \hat{n} \cdot \vec{S}_2 \vec{S}_1 \cdot \vec{v}_1 \hat{n} \cdot \vec{v}_1 + \frac{1}{7} \hat{n} \cdot \vec{S}_1 \vec{S}_2 \cdot \vec{v}_1 \hat{n} \cdot \vec{v}_1 - \right.$$

$$\left. \frac{1}{35} \vec{S}_1 \cdot \vec{v}_1 \vec{S}_2 \cdot \vec{v}_1 + \frac{1}{14} \hat{n} \cdot \vec{S}_1 \hat{n} \cdot \vec{S}_2 \vec{v}_1 \cdot \vec{v}_1 - \frac{1}{70} \vec{S}_1 \cdot \vec{S}_2 \vec{v}_1 \cdot \vec{v}_1 \right) \Bigg\}$$

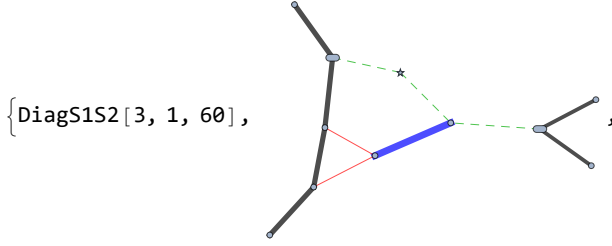

$$\begin{aligned} G^3 m_1^2 \Bigg( & \frac{\frac{1}{2} \vec{S}_1 \cdot \vec{S}_2 - \frac{1}{2} \hat{n} \cdot \vec{S}_1 \hat{n} \cdot \vec{S}_2}{r^3} + \frac{1}{r^4} \left( \frac{9}{2} \hat{n} \cdot \vec{S}_2 \hat{n} \cdot \vec{S}_1 \hat{n} \cdot \vec{v}_1 - \frac{1}{2} \hat{n} \cdot \vec{S}_1 \hat{n} \cdot \vec{S}_2 \hat{n} \cdot \vec{v}_1 - \right. \\ & \frac{17}{25} \vec{S}_1 \cdot \vec{S}_2 \hat{n} \cdot \vec{v}_1 - \frac{33}{25} \vec{S}_1 \cdot \vec{S}_2 \hat{n} \cdot \vec{v}_1 - 4 \hat{n} \cdot \vec{S}_1 \hat{n} \cdot \vec{S}_2 \hat{n} \cdot \vec{v}_2 + 2 \hat{n} \cdot \vec{v}_2 \vec{S}_1 \cdot \vec{S}_2 + \frac{11}{50} \hat{n} \cdot \vec{S}_2 \vec{S}_1 \cdot \vec{v}_1 + \\ & \left. \frac{1}{2} \hat{n} \cdot \vec{S}_2 \vec{S}_1 \cdot \vec{v}_2 - \frac{51}{50} \hat{n} \cdot \vec{S}_1 \vec{S}_2 \cdot \vec{v}_1 - \frac{18}{25} \hat{n} \cdot \vec{S}_2 \vec{S}_1 \cdot \vec{v}_1 + \frac{13}{25} \hat{n} \cdot \vec{S}_1 \vec{S}_2 \cdot \vec{v}_1 + \frac{1}{2} \hat{n} \cdot \vec{S}_1 \vec{S}_2 \cdot \vec{v}_2 \right) + \frac{1}{r^5} \\ & \left( -3 \hat{n} \cdot \vec{S}_1 \hat{n} \cdot \vec{S}_2 (\hat{n} \cdot \vec{v}_1)^2 + \frac{103}{98} \vec{S}_1 \cdot \vec{S}_2 (\hat{n} \cdot \vec{v}_1)^2 + 36 \hat{n} \cdot \vec{S}_1 \hat{n} \cdot \vec{S}_2 \hat{n} \cdot \vec{v}_2 \hat{n} \cdot \vec{v}_1 - \frac{15}{2} \hat{n} \cdot \vec{v}_2 \vec{S}_1 \cdot \vec{S}_2 \hat{n} \cdot \vec{v}_1 + \right. \\ & \frac{33}{49} \hat{n} \cdot \vec{S}_2 \vec{S}_1 \cdot \vec{v}_1 \hat{n} \cdot \vec{v}_1 - \frac{9}{2} \hat{n} \cdot \vec{S}_2 \vec{S}_1 \cdot \vec{v}_2 \hat{n} \cdot \vec{v}_1 + \frac{59}{98} \hat{n} \cdot \vec{S}_1 \vec{S}_2 \cdot \vec{v}_1 \hat{n} \cdot \vec{v}_1 - \frac{9}{2} \hat{n} \cdot \vec{S}_1 \vec{S}_2 \cdot \vec{v}_2 \hat{n} \cdot \vec{v}_1 - \\ & \frac{1}{7} \hat{n} \times \vec{S}_1 \cdot \vec{v}_1 \hat{n} \times \vec{S}_2 \cdot \vec{v}_1 - \frac{9}{2} \hat{n} \cdot \vec{S}_2 \hat{n} \cdot \vec{v}_2 \vec{S}_1 \cdot \vec{v}_1 - 6 \hat{n} \cdot \vec{S}_1 \hat{n} \cdot \vec{v}_2 \vec{S}_2 \cdot \vec{v}_1 - \frac{239 \vec{S}_1 \cdot \vec{v}_1 \vec{S}_2 \cdot \vec{v}_1}{2450} + \frac{51}{50} \vec{S}_1 \cdot \vec{v}_2 \vec{S}_2 \cdot \vec{v}_1 + \\ & \left. \frac{18}{25} \vec{S}_1 \cdot \vec{v}_1 \vec{S}_2 \cdot \vec{v}_2 - \frac{37}{98} \hat{n} \cdot \vec{S}_1 \hat{n} \cdot \vec{S}_2 \vec{v}_1 \cdot \vec{v}_1 + \frac{334 \vec{S}_1 \cdot \vec{S}_2 \vec{v}_1 \cdot \vec{v}_1}{1225} - \frac{9}{2} \hat{n} \cdot \vec{S}_1 \hat{n} \cdot \vec{S}_2 \vec{v}_1 \cdot \vec{v}_2 + \frac{33}{25} \vec{S}_1 \cdot \vec{S}_2 \vec{v}_1 \cdot \vec{v}_2 \right) + \\ & \left( \frac{\frac{3}{2} \hat{n} \cdot \vec{S}_1 \hat{n} \cdot \vec{S}_2 - \frac{1}{2} \vec{S}_1 \cdot \vec{S}_2}{r^3} + \frac{1}{r^4} \left( -\frac{9}{2} \hat{n} \cdot \vec{S}_2 \hat{n} \cdot \vec{S}_1 \hat{n} \cdot \vec{v}_1 - 3 \hat{n} \cdot \vec{S}_1 \hat{n} \cdot \vec{S}_2 \hat{n} \cdot \vec{v}_1 + \frac{3}{5} \vec{S}_1 \cdot \vec{S}_2 \hat{n} \cdot \vec{v}_1 + \right. \right. \\ & \frac{9}{10} \vec{S}_1 \cdot \vec{S}_2 \hat{n} \cdot \vec{v}_1 + \frac{15}{2} \hat{n} \cdot \vec{S}_1 \hat{n} \cdot \vec{S}_2 \hat{n} \cdot \vec{v}_2 - \frac{3}{2} \hat{n} \cdot \vec{v}_2 \vec{S}_1 \cdot \vec{S}_2 + \frac{3}{5} \hat{n} \cdot \vec{S}_2 \vec{S}_1 \cdot \vec{v}_1 - \\ & \left. \frac{3}{2} \hat{n} \cdot \vec{S}_2 \vec{S}_1 \cdot \vec{v}_2 + \frac{9}{10} \hat{n} \cdot \vec{S}_1 \vec{S}_2 \cdot \vec{v}_1 + \frac{9}{10} \hat{n} \cdot \vec{S}_2 \vec{S}_1 \cdot \vec{v}_1 + \frac{3}{5} \hat{n} \cdot \vec{S}_1 \vec{S}_2 \cdot \vec{v}_1 - \frac{3}{2} \hat{n} \cdot \vec{S}_1 \vec{S}_2 \cdot \vec{v}_2 \right) + \frac{1}{r^5} \\ & \left( \frac{9}{2} \hat{n} \cdot \vec{S}_1 \hat{n} \cdot \vec{S}_2 (\hat{n} \cdot \vec{v}_1)^2 - \frac{9}{14} \vec{S}_1 \cdot \vec{S}_2 (\hat{n} \cdot \vec{v}_1)^2 - \frac{63}{2} \hat{n} \cdot \vec{S}_1 \hat{n} \cdot \vec{S}_2 \hat{n} \cdot \vec{v}_2 \hat{n} \cdot \vec{v}_1 + \frac{9}{2} \hat{n} \cdot \vec{v}_2 \vec{S}_1 \cdot \vec{S}_2 \hat{n} \cdot \vec{v}_1 - \right. \\ & \frac{9}{7} \hat{n} \cdot \vec{S}_2 \vec{S}_1 \cdot \vec{v}_1 \hat{n} \cdot \vec{v}_1 + \frac{9}{2} \hat{n} \cdot \vec{S}_2 \vec{S}_1 \cdot \vec{v}_2 \hat{n} \cdot \vec{v}_1 - \frac{9}{7} \hat{n} \cdot \vec{S}_1 \vec{S}_2 \cdot \vec{v}_1 \hat{n} \cdot \vec{v}_1 + \frac{9}{2} \hat{n} \cdot \vec{S}_1 \vec{S}_2 \cdot \vec{v}_2 \hat{n} \cdot \vec{v}_1 + \\ & \frac{9}{2} \hat{n} \cdot \vec{S}_2 \hat{n} \cdot \vec{v}_2 \vec{S}_1 \cdot \vec{v}_1 + \frac{9}{2} \hat{n} \cdot \vec{S}_1 \hat{n} \cdot \vec{v}_2 \vec{S}_2 \cdot \vec{v}_1 + \frac{9}{35} \vec{S}_1 \cdot \vec{v}_1 \vec{S}_2 \cdot \vec{v}_1 - \frac{9}{10} \vec{S}_1 \cdot \vec{v}_2 \vec{S}_2 \cdot \vec{v}_1 - \frac{9}{10} \vec{S}_1 \cdot \vec{v}_1 \vec{S}_2 \cdot \vec{v}_2 - \\ & \left. \frac{9}{14} \hat{n} \cdot \vec{S}_1 \hat{n} \cdot \vec{S}_2 \vec{v}_1 \cdot \vec{v}_1 + \frac{9}{70} \vec{S}_1 \cdot \vec{S}_2 \vec{v}_1 \cdot \vec{v}_1 + \frac{9}{2} \hat{n} \cdot \vec{S}_1 \hat{n} \cdot \vec{S}_2 \vec{v}_1 \cdot \vec{v}_2 - \frac{9}{10} \vec{S}_1 \cdot \vec{S}_2 \vec{v}_1 \cdot \vec{v}_2 \right) \log \left( \frac{r}{R_0} \right) + \\ & \frac{1}{\epsilon_d} \left( \frac{\frac{1}{6} \vec{S}_1 \cdot \vec{S}_2 - \frac{1}{2} \hat{n} \cdot \vec{S}_1 \hat{n} \cdot \vec{S}_2}{r^3} + \frac{1}{r^4} \left( \frac{3}{2} \hat{n} \cdot \vec{S}_2 \hat{n} \cdot \vec{S}_1 \hat{n} \cdot \vec{v}_1 + \hat{n} \cdot \vec{S}_1 \hat{n} \cdot \vec{S}_2 \hat{n} \cdot \vec{v}_1 - \frac{1}{5} \vec{S}_1 \cdot \vec{S}_2 \hat{n} \cdot \vec{v}_1 - \right. \right. \\ & \left. \frac{3}{10} \vec{S}_1 \cdot \vec{S}_2 \hat{n} \cdot \vec{v}_1 - \frac{5}{2} \hat{n} \cdot \vec{S}_1 \hat{n} \cdot \vec{S}_2 \hat{n} \cdot \vec{v}_2 + \frac{1}{2} \hat{n} \cdot \vec{v}_2 \vec{S}_1 \cdot \vec{S}_2 - \frac{1}{5} \hat{n} \cdot \vec{S}_2 \vec{S}_1 \cdot \vec{v}_1 + \frac{1}{2} \hat{n} \cdot \vec{S}_2 \vec{S}_1 \cdot \vec{v}_2 - \right. \end{aligned}$$



$$\left. \begin{aligned} & \frac{3}{10} \hat{n} \cdot \vec{S}_1 \vec{S}_2 \cdot \vec{v}_1 - \frac{3}{10} \hat{n} \cdot \vec{S}_2 \vec{S}_1 \cdot \vec{v}_1 - \frac{1}{5} \hat{n} \cdot \vec{S}_1 \vec{S}_2 \cdot \vec{v}_1 + \frac{1}{2} \hat{n} \cdot \vec{S}_1 \vec{S}_2 \cdot \vec{v}_2 \Big) + \frac{1}{r^5} \\ & \left( -\frac{3}{2} \hat{n} \cdot \vec{S}_1 \hat{n} \cdot \vec{S}_2 (\hat{n} \cdot \vec{v}_1)^2 + \frac{3}{14} \vec{S}_1 \cdot \vec{S}_2 (\hat{n} \cdot \vec{v}_1)^2 + \frac{21}{2} \hat{n} \cdot \vec{S}_1 \hat{n} \cdot \vec{S}_2 \hat{n} \cdot \vec{v}_2 \hat{n} \cdot \vec{v}_1 - \frac{3}{2} \hat{n} \cdot \vec{v}_2 \vec{S}_1 \cdot \vec{S}_2 \hat{n} \cdot \vec{v}_1 + \right. \\ & \quad \frac{3}{7} \hat{n} \cdot \vec{S}_2 \vec{S}_1 \cdot \vec{v}_1 \hat{n} \cdot \vec{v}_1 - \frac{3}{2} \hat{n} \cdot \vec{S}_2 \vec{S}_1 \cdot \vec{v}_2 \hat{n} \cdot \vec{v}_1 + \frac{3}{7} \hat{n} \cdot \vec{S}_1 \vec{S}_2 \cdot \vec{v}_1 \hat{n} \cdot \vec{v}_1 - \frac{3}{2} \hat{n} \cdot \vec{S}_1 \vec{S}_2 \cdot \vec{v}_2 \hat{n} \cdot \vec{v}_1 - \\ & \quad \frac{3}{2} \hat{n} \cdot \vec{S}_2 \hat{n} \cdot \vec{v}_2 \vec{S}_1 \cdot \vec{v}_1 - \frac{3}{2} \hat{n} \cdot \vec{S}_1 \hat{n} \cdot \vec{v}_2 \vec{S}_2 \cdot \vec{v}_1 - \frac{3}{35} \vec{S}_1 \cdot \vec{v}_1 \vec{S}_2 \cdot \vec{v}_1 + \frac{3}{10} \vec{S}_1 \cdot \vec{v}_2 \vec{S}_2 \cdot \vec{v}_1 + \frac{3}{10} \vec{S}_1 \cdot \vec{v}_1 \vec{S}_2 \cdot \vec{v}_2 + \\ & \quad \left. \frac{3}{14} \hat{n} \cdot \vec{S}_1 \hat{n} \cdot \vec{S}_2 \vec{v}_1 \cdot \vec{v}_1 - \frac{3}{70} \vec{S}_1 \cdot \vec{S}_2 \vec{v}_1 \cdot \vec{v}_1 - \frac{3}{2} \hat{n} \cdot \vec{S}_1 \hat{n} \cdot \vec{S}_2 \vec{v}_1 \cdot \vec{v}_2 + \frac{3}{10} \vec{S}_1 \cdot \vec{S}_2 \vec{v}_1 \cdot \vec{v}_2 \right) \Bigg] \Bigg\} \end{aligned} \right.$$

$$\{\text{DiagS1S2}[3, 1, 61],$$

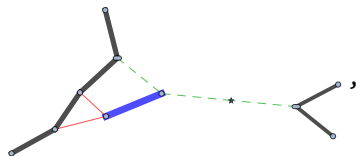

$$G^3 m_1^2 \left( \frac{\frac{49}{100} \hat{n} \cdot \vec{S}_1 \hat{n} \cdot \vec{S}_2 - \frac{23}{100} \vec{S}_1 \cdot \vec{S}_2}{r^3} + \frac{1}{r^4} \left( -\frac{11}{4} \hat{n} \cdot \vec{S}_2 \hat{n} \cdot \vec{S}_1 \hat{n} \cdot \vec{v}_1 + \frac{79}{100} \vec{S}_1 \cdot \vec{S}_2 \hat{n} \cdot \vec{v}_1 + \frac{11}{4} \hat{n} \cdot \vec{S}_1 \hat{n} \cdot \vec{S}_2 \hat{n} \cdot \vec{v}_2 - \right. \right. \\ \frac{79}{100} \hat{n} \cdot \vec{v}_2 \vec{S}_1 \cdot \vec{S}_2 - \frac{49}{100} \hat{n} \cdot \vec{S}_2 \vec{S}_1 \cdot \vec{v}_2 + \frac{49}{100} \hat{n} \cdot \vec{S}_1 \vec{S}_2 \cdot \vec{v}_1 + \frac{49}{100} \hat{n} \cdot \vec{S}_2 \vec{S}_1 \cdot \vec{v}_1 - \frac{49}{100} \hat{n} \cdot \vec{S}_1 \vec{S}_2 \cdot \vec{v}_2 \Big) + \\ \frac{1}{r^5} \left( -\frac{83}{4} \hat{n} \cdot \vec{S}_1 \hat{n} \cdot \vec{S}_2 \hat{n} \cdot \vec{v}_1 \hat{n} \cdot \vec{v}_2 + \frac{17}{4} \hat{n} \cdot \vec{v}_1 \vec{S}_1 \cdot \vec{S}_2 \hat{n} \cdot \vec{v}_2 + \frac{11}{4} \hat{n} \cdot \vec{S}_2 \vec{S}_1 \cdot \vec{v}_1 \hat{n} \cdot \vec{v}_2 + \right. \\ \frac{11}{4} \hat{n} \cdot \vec{S}_1 \vec{S}_2 \cdot \vec{v}_1 \hat{n} \cdot \vec{v}_2 + \frac{11}{4} \hat{n} \cdot \vec{S}_2 \hat{n} \cdot \vec{v}_1 \vec{S}_1 \cdot \vec{v}_2 - \frac{49}{100} \vec{S}_1 \cdot \vec{v}_2 \vec{S}_2 \cdot \vec{v}_1 + \\ \frac{11}{4} \hat{n} \cdot \vec{S}_1 \hat{n} \cdot \vec{v}_1 \vec{S}_2 \cdot \vec{v}_2 - \frac{49}{100} \vec{S}_1 \cdot \vec{v}_1 \vec{S}_2 \cdot \vec{v}_2 + \frac{11}{4} \hat{n} \cdot \vec{S}_1 \hat{n} \cdot \vec{S}_2 \vec{v}_1 \cdot \vec{v}_2 - \frac{79}{100} \vec{S}_1 \cdot \vec{S}_2 \vec{v}_1 \cdot \vec{v}_2 \Big) + \\ \left. \left( \frac{\frac{1}{10} \vec{S}_1 \cdot \vec{S}_2 - \frac{3}{10} \hat{n} \cdot \vec{S}_1 \hat{n} \cdot \vec{S}_2}{r^3} + \frac{1}{r^4} \left( \frac{3}{2} \hat{n} \cdot \vec{S}_2 \hat{n} \cdot \vec{S}_1 \hat{n} \cdot \vec{v}_1 - \frac{3}{10} \vec{S}_1 \cdot \vec{S}_2 \hat{n} \cdot \vec{v}_1 - \frac{3}{2} \hat{n} \cdot \vec{S}_1 \hat{n} \cdot \vec{S}_2 \hat{n} \cdot \vec{v}_2 + \frac{3}{10} \hat{n} \cdot \vec{v}_2 \vec{S}_1 \cdot \vec{S}_2 + \right. \right. \\ \frac{3}{10} \hat{n} \cdot \vec{S}_2 \vec{S}_1 \cdot \vec{v}_2 - \frac{3}{10} \hat{n} \cdot \vec{S}_1 \vec{S}_2 \cdot \vec{v}_1 - \frac{3}{10} \hat{n} \cdot \vec{S}_2 \vec{S}_1 \cdot \vec{v}_1 + \frac{3}{10} \hat{n} \cdot \vec{S}_1 \vec{S}_2 \cdot \vec{v}_2 \Big) + \frac{1}{r^5} \left( \frac{21}{2} \hat{n} \cdot \vec{S}_1 \hat{n} \cdot \vec{S}_2 \hat{n} \cdot \vec{v}_1 \hat{n} \cdot \vec{v}_2 - \right. \\ \frac{3}{2} \hat{n} \cdot \vec{v}_1 \vec{S}_1 \cdot \vec{S}_2 \hat{n} \cdot \vec{v}_2 - \frac{3}{2} \hat{n} \cdot \vec{S}_2 \vec{S}_1 \cdot \vec{v}_1 \hat{n} \cdot \vec{v}_2 - \frac{3}{2} \hat{n} \cdot \vec{S}_1 \vec{S}_2 \cdot \vec{v}_1 \hat{n} \cdot \vec{v}_2 - \frac{3}{2} \hat{n} \cdot \vec{S}_2 \hat{n} \cdot \vec{v}_1 \vec{S}_1 \cdot \vec{v}_2 + \frac{3}{10} \vec{S}_1 \cdot \vec{v}_2 \vec{S}_2 \cdot \vec{v}_1 - \\ \frac{3}{2} \hat{n} \cdot \vec{S}_1 \hat{n} \cdot \vec{v}_1 \vec{S}_2 \cdot \vec{v}_2 + \frac{3}{10} \vec{S}_1 \cdot \vec{v}_1 \vec{S}_2 \cdot \vec{v}_2 - \frac{3}{2} \hat{n} \cdot \vec{S}_1 \hat{n} \cdot \vec{S}_2 \vec{v}_1 \cdot \vec{v}_2 + \frac{3}{10} \vec{S}_1 \cdot \vec{S}_2 \vec{v}_1 \cdot \vec{v}_2 \Big) \right) \log \left( \frac{r}{R_\theta} \right) + \frac{1}{\epsilon_d} \\ \left. \left( \frac{\frac{1}{10} \hat{n} \cdot \vec{S}_1 \hat{n} \cdot \vec{S}_2 - \frac{1}{30} \vec{S}_1 \cdot \vec{S}_2}{r^3} + \frac{1}{r^4} \left( -\frac{1}{2} \hat{n} \cdot \vec{S}_2 \hat{n} \cdot \vec{S}_1 \hat{n} \cdot \vec{v}_1 + \frac{1}{10} \vec{S}_1 \cdot \vec{S}_2 \hat{n} \cdot \vec{v}_1 + \frac{1}{2} \hat{n} \cdot \vec{S}_1 \hat{n} \cdot \vec{S}_2 \hat{n} \cdot \vec{v}_2 - \frac{1}{10} \hat{n} \cdot \vec{v}_2 \vec{S}_1 \cdot \vec{S}_2 - \right. \right. \\ \frac{1}{10} \hat{n} \cdot \vec{S}_2 \vec{S}_1 \cdot \vec{v}_2 + \frac{1}{10} \hat{n} \cdot \vec{S}_1 \vec{S}_2 \cdot \vec{v}_1 + \frac{1}{10} \hat{n} \cdot \vec{S}_2 \vec{S}_1 \cdot \vec{v}_1 - \frac{1}{10} \hat{n} \cdot \vec{S}_1 \vec{S}_2 \cdot \vec{v}_2 \Big) + \frac{1}{r^5} \left( -\frac{7}{2} \hat{n} \cdot \vec{S}_1 \hat{n} \cdot \vec{S}_2 \hat{n} \cdot \vec{v}_1 \hat{n} \cdot \vec{v}_2 + \right. \\ \frac{1}{2} \hat{n} \cdot \vec{v}_1 \vec{S}_1 \cdot \vec{S}_2 \hat{n} \cdot \vec{v}_2 + \frac{1}{2} \hat{n} \cdot \vec{S}_2 \vec{S}_1 \cdot \vec{v}_1 \hat{n} \cdot \vec{v}_2 + \frac{1}{2} \hat{n} \cdot \vec{S}_1 \vec{S}_2 \cdot \vec{v}_1 \hat{n} \cdot \vec{v}_2 + \frac{1}{2} \hat{n} \cdot \vec{S}_2 \hat{n} \cdot \vec{v}_1 \vec{S}_1 \cdot \vec{v}_2 - \\ \frac{1}{10} \vec{S}_1 \cdot \vec{v}_2 \vec{S}_2 \cdot \vec{v}_1 + \frac{1}{2} \hat{n} \cdot \vec{S}_1 \hat{n} \cdot \vec{v}_1 \vec{S}_2 \cdot \vec{v}_2 - \frac{1}{10} \vec{S}_1 \cdot \vec{v}_1 \vec{S}_2 \cdot \vec{v}_2 + \frac{1}{2} \hat{n} \cdot \vec{S}_1 \hat{n} \cdot \vec{S}_2 \vec{v}_1 \cdot \vec{v}_2 - \frac{1}{10} \vec{S}_1 \cdot \vec{S}_2 \vec{v}_1 \cdot \vec{v}_2 \Big) \right) \Bigg\}$$

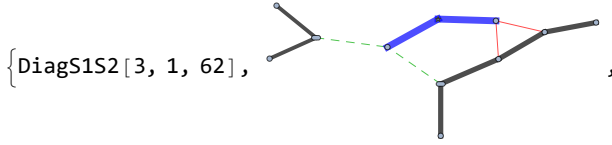

$$\begin{aligned}
 G^3 m_1^2 & \left( \frac{1}{r^4} \left( -\frac{5}{2} \hat{n} \cdot \vec{S}_2 \hat{n} \cdot \vec{S}_1 \hat{n} \cdot \vec{v}_1 - \frac{5}{2} \hat{n} \cdot \vec{S}_1 \hat{n} \cdot \vec{S}_2 \hat{n} \cdot \vec{v}_1 + \frac{16}{25} \vec{S}_1 \cdot \vec{S}_2 \hat{n} \cdot \vec{v}_1 + \right. \right. \\
 & \left. \frac{16}{25} \vec{S}_1 \cdot \vec{S}_2 \hat{n} \cdot \vec{v}_1 + \frac{11}{25} \hat{n} \cdot \vec{S}_2 \vec{S}_1 \cdot \vec{v}_1 + \frac{27}{50} \hat{n} \cdot \vec{S}_1 \vec{S}_2 \cdot \vec{v}_1 + \frac{11}{25} \hat{n} \cdot \vec{S}_2 \vec{S}_1 \cdot \vec{v}_1 + \frac{27}{50} \hat{n} \cdot \vec{S}_1 \vec{S}_2 \cdot \vec{v}_1 \right) + \frac{1}{r^5} \\
 & \left( \frac{50}{3} \hat{n} \cdot \vec{S}_1 \hat{n} \cdot \vec{S}_2 (\hat{n} \cdot \vec{v}_1)^2 - \frac{943}{294} \vec{S}_1 \cdot \vec{S}_2 (\hat{n} \cdot \vec{v}_1)^2 - 19 \hat{n} \cdot \vec{S}_1 \hat{n} \cdot \vec{S}_2 \hat{n} \cdot \vec{v}_2 \hat{n} \cdot \vec{v}_1 + \frac{7}{2} \hat{n} \cdot \vec{v}_2 \vec{S}_1 \cdot \vec{S}_2 \hat{n} \cdot \vec{v}_1 - \right. \\
 & \frac{628}{147} \hat{n} \cdot \vec{S}_2 \vec{S}_1 \cdot \vec{v}_1 \hat{n} \cdot \vec{v}_1 + \frac{5}{2} \hat{n} \cdot \vec{S}_2 \vec{S}_1 \cdot \vec{v}_2 \hat{n} \cdot \vec{v}_1 - \frac{1445}{294} \hat{n} \cdot \vec{S}_1 \vec{S}_2 \cdot \vec{v}_1 \hat{n} \cdot \vec{v}_1 + \frac{5}{2} \hat{n} \cdot \vec{S}_1 \vec{S}_2 \cdot \vec{v}_2 \hat{n} \cdot \vec{v}_1 - \\
 & \frac{2}{7} \hat{n} \times \vec{S}_1 \cdot \vec{v}_1 \hat{n} \times \vec{S}_2 \cdot \vec{v}_1 + \frac{5}{2} \hat{n} \cdot \vec{S}_2 \hat{n} \cdot \vec{v}_2 \vec{S}_1 \cdot \vec{v}_1 + 3 \hat{n} \cdot \vec{S}_1 \hat{n} \cdot \vec{v}_2 \vec{S}_2 \cdot \vec{v}_1 + \frac{5797 \vec{S}_1 \cdot \vec{v}_1 \vec{S}_2 \cdot \vec{v}_1}{7350} - \frac{27}{50} \vec{S}_1 \cdot \vec{v}_2 \vec{S}_2 \cdot \vec{v}_1 - \\
 & \left. \frac{11}{25} \vec{S}_1 \cdot \vec{v}_1 \vec{S}_2 \cdot \vec{v}_2 - \frac{377}{147} \hat{n} \cdot \vec{S}_1 \hat{n} \cdot \vec{S}_2 \vec{v}_1 \cdot \vec{v}_1 + \frac{6521 \vec{S}_1 \cdot \vec{S}_2 \vec{v}_1 \cdot \vec{v}_1}{7350} + \frac{5}{2} \hat{n} \cdot \vec{S}_1 \hat{n} \cdot \vec{S}_2 \vec{v}_1 \cdot \vec{v}_2 - \frac{16}{25} \vec{S}_1 \cdot \vec{S}_2 \vec{v}_1 \cdot \vec{v}_2 \right) + \\
 & \left( \frac{1}{r^4} \left( \frac{3}{2} \hat{n} \cdot \vec{S}_2 \hat{n} \cdot \vec{S}_1 \hat{n} \cdot \vec{v}_1 + \frac{3}{2} \hat{n} \cdot \vec{S}_1 \hat{n} \cdot \vec{S}_2 \hat{n} \cdot \vec{v}_1 - \frac{3}{10} \vec{S}_1 \cdot \vec{S}_2 \hat{n} \cdot \vec{v}_1 - \frac{3}{10} \vec{S}_1 \cdot \vec{S}_2 \hat{n} \cdot \vec{v}_1 - \right. \right. \\
 & \left. \frac{3}{10} \hat{n} \cdot \vec{S}_2 \vec{S}_1 \cdot \vec{v}_1 - \frac{3}{10} \hat{n} \cdot \vec{S}_1 \vec{S}_2 \cdot \vec{v}_1 - \frac{3}{10} \hat{n} \cdot \vec{S}_2 \vec{S}_1 \cdot \vec{v}_1 - \frac{3}{10} \hat{n} \cdot \vec{S}_1 \vec{S}_2 \cdot \vec{v}_1 \right) + \frac{1}{r^5} \\
 & \left( -12 \hat{n} \cdot \vec{S}_1 \hat{n} \cdot \vec{S}_2 (\hat{n} \cdot \vec{v}_1)^2 + \frac{12}{7} \vec{S}_1 \cdot \vec{S}_2 (\hat{n} \cdot \vec{v}_1)^2 + \frac{21}{2} \hat{n} \cdot \vec{S}_1 \hat{n} \cdot \vec{S}_2 \hat{n} \cdot \vec{v}_2 \hat{n} \cdot \vec{v}_1 - \frac{3}{2} \hat{n} \cdot \vec{v}_2 \vec{S}_1 \cdot \vec{S}_2 \hat{n} \cdot \vec{v}_1 + \right. \\
 & \frac{24}{7} \hat{n} \cdot \vec{S}_2 \vec{S}_1 \cdot \vec{v}_1 \hat{n} \cdot \vec{v}_1 - \frac{3}{2} \hat{n} \cdot \vec{S}_2 \vec{S}_1 \cdot \vec{v}_2 \hat{n} \cdot \vec{v}_1 + \frac{24}{7} \hat{n} \cdot \vec{S}_1 \vec{S}_2 \cdot \vec{v}_1 \hat{n} \cdot \vec{v}_1 - \frac{3}{2} \hat{n} \cdot \vec{S}_1 \vec{S}_2 \cdot \vec{v}_2 \hat{n} \cdot \vec{v}_1 - \\
 & \frac{3}{2} \hat{n} \cdot \vec{S}_2 \hat{n} \cdot \vec{v}_2 \vec{S}_1 \cdot \vec{v}_1 - \frac{3}{2} \hat{n} \cdot \vec{S}_1 \hat{n} \cdot \vec{v}_2 \vec{S}_2 \cdot \vec{v}_1 - \frac{24}{35} \vec{S}_1 \cdot \vec{v}_1 \vec{S}_2 \cdot \vec{v}_1 + \frac{3}{10} \vec{S}_1 \cdot \vec{v}_2 \vec{S}_2 \cdot \vec{v}_1 + \frac{3}{10} \vec{S}_1 \cdot \vec{v}_1 \vec{S}_2 \cdot \vec{v}_2 + \\
 & \left. \frac{12}{7} \hat{n} \cdot \vec{S}_1 \hat{n} \cdot \vec{S}_2 \vec{v}_1 \cdot \vec{v}_1 - \frac{12}{35} \vec{S}_1 \cdot \vec{S}_2 \vec{v}_1 \cdot \vec{v}_1 - \frac{3}{2} \hat{n} \cdot \vec{S}_1 \hat{n} \cdot \vec{S}_2 \vec{v}_1 \cdot \vec{v}_2 + \frac{3}{10} \vec{S}_1 \cdot \vec{S}_2 \vec{v}_1 \cdot \vec{v}_2 \right) \log \left( \frac{r}{R_0} \right) + \\
 & \frac{1}{\epsilon_d} \left( \frac{1}{r^4} \left( -\frac{1}{2} \hat{n} \cdot \vec{S}_2 \hat{n} \cdot \vec{S}_1 \hat{n} \cdot \vec{v}_1 - \frac{1}{2} \hat{n} \cdot \vec{S}_1 \hat{n} \cdot \vec{S}_2 \hat{n} \cdot \vec{v}_1 + \frac{1}{10} \vec{S}_1 \cdot \vec{S}_2 \hat{n} \cdot \vec{v}_1 + \frac{1}{10} \vec{S}_1 \cdot \vec{S}_2 \hat{n} \cdot \vec{v}_1 + \right. \right. \\
 & \left. \frac{1}{10} \hat{n} \cdot \vec{S}_2 \vec{S}_1 \cdot \vec{v}_1 + \frac{1}{10} \hat{n} \cdot \vec{S}_1 \vec{S}_2 \cdot \vec{v}_1 + \frac{1}{10} \hat{n} \cdot \vec{S}_2 \vec{S}_1 \cdot \vec{v}_1 + \frac{1}{10} \hat{n} \cdot \vec{S}_1 \vec{S}_2 \cdot \vec{v}_1 \right) + \frac{1}{r^5} \\
 & \left( 4 \hat{n} \cdot \vec{S}_1 \hat{n} \cdot \vec{S}_2 (\hat{n} \cdot \vec{v}_1)^2 - \frac{4}{7} \vec{S}_1 \cdot \vec{S}_2 (\hat{n} \cdot \vec{v}_1)^2 - \frac{7}{2} \hat{n} \cdot \vec{S}_1 \hat{n} \cdot \vec{S}_2 \hat{n} \cdot \vec{v}_2 \hat{n} \cdot \vec{v}_1 + \frac{1}{2} \hat{n} \cdot \vec{v}_2 \vec{S}_1 \cdot \vec{S}_2 \hat{n} \cdot \vec{v}_1 - \right. \\
 & \frac{8}{7} \hat{n} \cdot \vec{S}_2 \vec{S}_1 \cdot \vec{v}_1 \hat{n} \cdot \vec{v}_1 + \frac{1}{2} \hat{n} \cdot \vec{S}_2 \vec{S}_1 \cdot \vec{v}_2 \hat{n} \cdot \vec{v}_1 - \frac{8}{7} \hat{n} \cdot \vec{S}_1 \vec{S}_2 \cdot \vec{v}_1 \hat{n} \cdot \vec{v}_1 + \frac{1}{2} \hat{n} \cdot \vec{S}_1 \vec{S}_2 \cdot \vec{v}_2 \hat{n} \cdot \vec{v}_1 + \\
 & \frac{1}{2} \hat{n} \cdot \vec{S}_2 \hat{n} \cdot \vec{v}_2 \vec{S}_1 \cdot \vec{v}_1 + \frac{1}{2} \hat{n} \cdot \vec{S}_1 \hat{n} \cdot \vec{v}_2 \vec{S}_2 \cdot \vec{v}_1 + \frac{8}{35} \vec{S}_1 \cdot \vec{v}_1 \vec{S}_2 \cdot \vec{v}_1 - \frac{1}{10} \vec{S}_1 \cdot \vec{v}_2 \vec{S}_2 \cdot \vec{v}_1 - \frac{1}{10} \vec{S}_1 \cdot \vec{v}_1 \vec{S}_2 \cdot \vec{v}_2 - \\
 & \left. \left. \frac{4}{7} \hat{n} \cdot \vec{S}_1 \hat{n} \cdot \vec{S}_2 \vec{v}_1 \cdot \vec{v}_1 + \frac{4}{35} \vec{S}_1 \cdot \vec{S}_2 \vec{v}_1 \cdot \vec{v}_1 + \frac{1}{2} \hat{n} \cdot \vec{S}_1 \hat{n} \cdot \vec{S}_2 \vec{v}_1 \cdot \vec{v}_2 - \frac{1}{10} \vec{S}_1 \cdot \vec{S}_2 \vec{v}_1 \cdot \vec{v}_2 \right) \right) \Bigg\}
 \end{aligned}$$

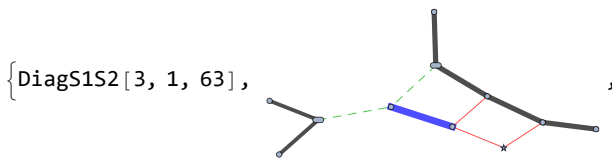

$$G^3 m_1^2 \left( \frac{1}{r^4} \left( -\frac{25}{2} \hat{n} \cdot \vec{S}_2 \hat{n} \cdot \vec{S}_1 \hat{n} \cdot \vec{v}_1 - \frac{25}{2} \hat{n} \cdot \vec{S}_1 \hat{n} \cdot \vec{S}_2 \hat{n} \cdot \vec{v}_1 + \frac{163}{50} \vec{S}_1 \cdot \vec{S}_2 \hat{n} \cdot \vec{v}_1 + \right. \right.$$

$$\begin{aligned}
& \left( \frac{163}{50} \vec{S}_1 \cdot \vec{S}_2 \hat{n} \cdot \vec{v}_1 + \frac{49}{25} \hat{n} \cdot \vec{S}_2 \vec{S}_1 \cdot \vec{v}_1 + \frac{84}{25} \hat{n} \cdot \vec{S}_1 \vec{S}_2 \cdot \vec{v}_1 + \frac{49}{25} \hat{n} \cdot \vec{S}_2 \vec{S}_1 \cdot \vec{v}_1 + \frac{84}{25} \hat{n} \cdot \vec{S}_1 \vec{S}_2 \cdot \vec{v}_1 \right) + \frac{1}{r^5} \\
& \left( \frac{653}{6} \hat{n} \cdot \vec{S}_1 \hat{n} \cdot \vec{S}_2 (\hat{n} \cdot \vec{v}_1)^2 - \frac{6329}{294} \vec{S}_1 \cdot \vec{S}_2 (\hat{n} \cdot \vec{v}_1)^2 - 101 \hat{n} \cdot \vec{S}_1 \hat{n} \cdot \vec{S}_2 \hat{n} \cdot \vec{v}_2 \hat{n} \cdot \vec{v}_1 + 19 \hat{n} \cdot \vec{v}_2 \vec{S}_1 \cdot \vec{S}_2 \hat{n} \cdot \vec{v}_1 - \right. \\
& \frac{3914}{147} \hat{n} \cdot \vec{S}_2 \vec{S}_1 \cdot \vec{v}_1 \hat{n} \cdot \vec{v}_1 + \frac{25}{2} \hat{n} \cdot \vec{S}_2 \vec{S}_1 \cdot \vec{v}_2 \hat{n} \cdot \vec{v}_1 - \frac{5006}{147} \hat{n} \cdot \vec{S}_1 \vec{S}_2 \cdot \vec{v}_1 \hat{n} \cdot \vec{v}_1 + \frac{25}{2} \hat{n} \cdot \vec{S}_1 \vec{S}_2 \cdot \vec{v}_2 \hat{n} \cdot \vec{v}_1 - \\
& \frac{6}{7} \hat{n} \times \vec{S}_1 \cdot \vec{v}_1 \hat{n} \times \vec{S}_2 \cdot \vec{v}_1 + \frac{25}{2} \hat{n} \cdot \vec{S}_2 \hat{n} \cdot \vec{v}_2 \vec{S}_1 \cdot \vec{v}_1 + \frac{39}{2} \hat{n} \cdot \vec{S}_1 \hat{n} \cdot \vec{v}_2 \vec{S}_2 \cdot \vec{v}_1 + \frac{19801 \vec{S}_1 \cdot \vec{v}_1 \vec{S}_2 \cdot \vec{v}_1}{3675} - \frac{84}{25} \vec{S}_1 \cdot \vec{v}_2 \vec{S}_2 \cdot \vec{v}_1 - \\
& \left. \frac{49}{25} \vec{S}_1 \cdot \vec{v}_1 \vec{S}_2 \cdot \vec{v}_2 - \frac{2146}{147} \hat{n} \cdot \vec{S}_1 \hat{n} \cdot \vec{S}_2 \vec{v}_1 \cdot \vec{v}_1 + \frac{16988 \vec{S}_1 \cdot \vec{S}_2 \vec{v}_1 \cdot \vec{v}_1}{3675} + \frac{25}{2} \hat{n} \cdot \vec{S}_1 \hat{n} \cdot \vec{S}_2 \vec{v}_1 \cdot \vec{v}_2 - \frac{163}{50} \vec{S}_1 \cdot \vec{S}_2 \vec{v}_1 \cdot \vec{v}_2 \right) + \\
& \left( \frac{1}{r^4} \left( \frac{27}{2} \hat{n} \cdot \vec{S}_2 \hat{n} \cdot \vec{S}_1 \hat{n} \cdot \vec{v}_1 + \frac{27}{2} \hat{n} \cdot \vec{S}_1 \hat{n} \cdot \vec{S}_2 \hat{n} \cdot \vec{v}_1 - \frac{27}{10} \vec{S}_1 \cdot \vec{S}_2 \hat{n} \cdot \vec{v}_1 - \frac{27}{10} \vec{S}_1 \cdot \vec{S}_2 \hat{n} \cdot \vec{v}_1 - \right. \right. \\
& \left. \frac{27}{10} \hat{n} \cdot \vec{S}_2 \vec{S}_1 \cdot \vec{v}_1 - \frac{27}{10} \hat{n} \cdot \vec{S}_1 \vec{S}_2 \cdot \vec{v}_1 - \frac{27}{10} \hat{n} \cdot \vec{S}_2 \vec{S}_1 \cdot \vec{v}_1 - \frac{27}{10} \hat{n} \cdot \vec{S}_1 \vec{S}_2 \cdot \vec{v}_1 \right) + \frac{1}{r^5} \\
& \left( -\frac{219}{2} \hat{n} \cdot \vec{S}_1 \hat{n} \cdot \vec{S}_2 (\hat{n} \cdot \vec{v}_1)^2 + \frac{219}{14} \vec{S}_1 \cdot \vec{S}_2 (\hat{n} \cdot \vec{v}_1)^2 + \frac{189}{2} \hat{n} \cdot \vec{S}_1 \hat{n} \cdot \vec{S}_2 \hat{n} \cdot \vec{v}_2 \hat{n} \cdot \vec{v}_1 - \frac{27}{2} \hat{n} \cdot \vec{v}_2 \vec{S}_1 \cdot \vec{S}_2 \hat{n} \cdot \vec{v}_1 + \right. \\
& \frac{219}{7} \hat{n} \cdot \vec{S}_2 \vec{S}_1 \cdot \vec{v}_1 \hat{n} \cdot \vec{v}_1 - \frac{27}{2} \hat{n} \cdot \vec{S}_2 \vec{S}_1 \cdot \vec{v}_2 \hat{n} \cdot \vec{v}_1 + \frac{219}{7} \hat{n} \cdot \vec{S}_1 \vec{S}_2 \cdot \vec{v}_1 \hat{n} \cdot \vec{v}_1 - \frac{27}{2} \hat{n} \cdot \vec{S}_1 \vec{S}_2 \cdot \vec{v}_2 \hat{n} \cdot \vec{v}_1 - \\
& \frac{27}{2} \hat{n} \cdot \vec{S}_2 \hat{n} \cdot \vec{v}_2 \vec{S}_1 \cdot \vec{v}_1 - \frac{27}{2} \hat{n} \cdot \vec{S}_1 \hat{n} \cdot \vec{v}_2 \vec{S}_2 \cdot \vec{v}_1 - \frac{219}{35} \vec{S}_1 \cdot \vec{v}_1 \vec{S}_2 \cdot \vec{v}_1 + \frac{27}{10} \vec{S}_1 \cdot \vec{v}_2 \vec{S}_2 \cdot \vec{v}_1 + \frac{27}{10} \vec{S}_1 \cdot \vec{v}_1 \vec{S}_2 \cdot \vec{v}_2 + \\
& \left. \frac{219}{14} \hat{n} \cdot \vec{S}_1 \hat{n} \cdot \vec{S}_2 \vec{v}_1 \cdot \vec{v}_1 - \frac{219}{70} \vec{S}_1 \cdot \vec{S}_2 \vec{v}_1 \cdot \vec{v}_1 - \frac{27}{2} \hat{n} \cdot \vec{S}_1 \hat{n} \cdot \vec{S}_2 \vec{v}_1 \cdot \vec{v}_2 + \frac{27}{10} \vec{S}_1 \cdot \vec{S}_2 \vec{v}_1 \cdot \vec{v}_2 \right) \log \left( \frac{r}{R_0} \right) + \\
& \frac{1}{\epsilon_d} \left( \frac{1}{r^4} \left( -\frac{9}{2} \hat{n} \cdot \vec{S}_2 \hat{n} \cdot \vec{S}_1 \hat{n} \cdot \vec{v}_1 - \frac{9}{2} \hat{n} \cdot \vec{S}_1 \hat{n} \cdot \vec{S}_2 \hat{n} \cdot \vec{v}_1 + \frac{9}{10} \vec{S}_1 \cdot \vec{S}_2 \hat{n} \cdot \vec{v}_1 + \frac{9}{10} \vec{S}_1 \cdot \vec{S}_2 \hat{n} \cdot \vec{v}_1 + \right. \right. \\
& \left. \frac{9}{10} \hat{n} \cdot \vec{S}_2 \vec{S}_1 \cdot \vec{v}_1 + \frac{9}{10} \hat{n} \cdot \vec{S}_1 \vec{S}_2 \cdot \vec{v}_1 + \frac{9}{10} \hat{n} \cdot \vec{S}_2 \vec{S}_1 \cdot \vec{v}_1 + \frac{9}{10} \hat{n} \cdot \vec{S}_1 \vec{S}_2 \cdot \vec{v}_1 \right) + \frac{1}{r^5} \\
& \left( \frac{73}{2} \hat{n} \cdot \vec{S}_1 \hat{n} \cdot \vec{S}_2 (\hat{n} \cdot \vec{v}_1)^2 - \frac{73}{14} \vec{S}_1 \cdot \vec{S}_2 (\hat{n} \cdot \vec{v}_1)^2 - \frac{63}{2} \hat{n} \cdot \vec{S}_1 \hat{n} \cdot \vec{S}_2 \hat{n} \cdot \vec{v}_2 \hat{n} \cdot \vec{v}_1 + \frac{9}{2} \hat{n} \cdot \vec{v}_2 \vec{S}_1 \cdot \vec{S}_2 \hat{n} \cdot \vec{v}_1 - \right. \\
& \frac{73}{7} \hat{n} \cdot \vec{S}_2 \vec{S}_1 \cdot \vec{v}_1 \hat{n} \cdot \vec{v}_1 + \frac{9}{2} \hat{n} \cdot \vec{S}_2 \vec{S}_1 \cdot \vec{v}_2 \hat{n} \cdot \vec{v}_1 - \frac{73}{7} \hat{n} \cdot \vec{S}_1 \vec{S}_2 \cdot \vec{v}_1 \hat{n} \cdot \vec{v}_1 + \frac{9}{2} \hat{n} \cdot \vec{S}_1 \vec{S}_2 \cdot \vec{v}_2 \hat{n} \cdot \vec{v}_1 + \\
& \frac{9}{2} \hat{n} \cdot \vec{S}_2 \hat{n} \cdot \vec{v}_2 \vec{S}_1 \cdot \vec{v}_1 + \frac{9}{2} \hat{n} \cdot \vec{S}_1 \hat{n} \cdot \vec{v}_2 \vec{S}_2 \cdot \vec{v}_1 + \frac{73}{35} \vec{S}_1 \cdot \vec{v}_1 \vec{S}_2 \cdot \vec{v}_1 - \frac{9}{10} \vec{S}_1 \cdot \vec{v}_2 \vec{S}_2 \cdot \vec{v}_1 - \frac{9}{10} \vec{S}_1 \cdot \vec{v}_1 \vec{S}_2 \cdot \vec{v}_2 - \\
& \left. \left. \frac{73}{14} \hat{n} \cdot \vec{S}_1 \hat{n} \cdot \vec{S}_2 \vec{v}_1 \cdot \vec{v}_1 + \frac{73}{70} \vec{S}_1 \cdot \vec{S}_2 \vec{v}_1 \cdot \vec{v}_1 + \frac{9}{2} \hat{n} \cdot \vec{S}_1 \hat{n} \cdot \vec{S}_2 \vec{v}_1 \cdot \vec{v}_2 - \frac{9}{10} \vec{S}_1 \cdot \vec{S}_2 \vec{v}_1 \cdot \vec{v}_2 \right) \right) \Bigg\}
\end{aligned}$$

{DiagS1S2 [3, 2, 1],

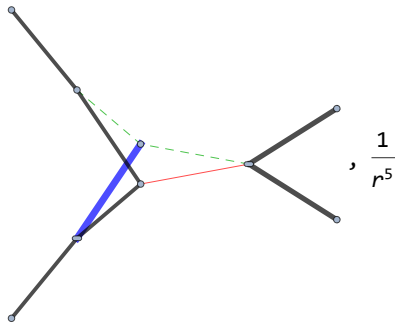

$$\begin{aligned}
& G^3 m_2^2 \left( 64 \hat{n} \times \vec{S}_1 \cdot \vec{v}_2 \hat{n} \times \vec{S}_2 \cdot \vec{v}_2 + 16 \vec{S}_1 \cdot \vec{S}_2 (\hat{n} \cdot \vec{v}_2)^2 - 16 \hat{n} \cdot \vec{S}_2 \hat{n} \cdot \vec{v}_2 \vec{S}_1 \cdot \vec{v}_2 + \right. \\
& \left. 48 \vec{v}_2 \cdot \vec{v}_2 \hat{n} \cdot \vec{S}_1 \hat{n} \cdot \vec{S}_2 + 20 \vec{S}_1 \cdot \vec{v}_2 \vec{S}_2 \cdot \vec{v}_2 - 44 \vec{S}_1 \cdot \vec{S}_2 \vec{v}_2 \cdot \vec{v}_2 \right) \Bigg\}
\end{aligned}$$

$\{\text{DiagS1S2}[3, 2, 2],$ 
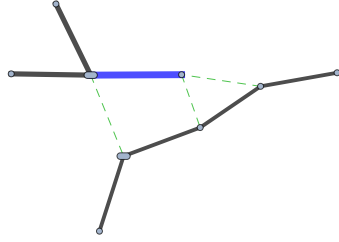
 $, \frac{1}{r^5}$ 

$$G^3 m_2^2 \left( -12 \hat{n} \times \vec{S}_1 \cdot \vec{v}_2 \hat{n} \times \vec{S}_2 \cdot \vec{v}_2 - 12 \vec{S}_1 \cdot \vec{S}_2 (\hat{n} \cdot \vec{v}_2)^2 + 12 \hat{n} \cdot \vec{S}_1 \hat{n} \cdot \vec{v}_2 \vec{S}_2 \cdot \vec{v}_2 - 14 \vec{v}_2 \cdot \vec{v}_2 \hat{n} \cdot \vec{S}_1 \hat{n} \cdot \vec{S}_2 - 8 \vec{S}_1 \cdot \vec{v}_2 \vec{S}_2 \cdot \vec{v}_2 + 14 \vec{S}_1 \cdot \vec{S}_2 \vec{v}_2 \cdot \vec{v}_2 \right) \}$$

 $\{\text{DiagS1S2}[3, 2, 3],$ 
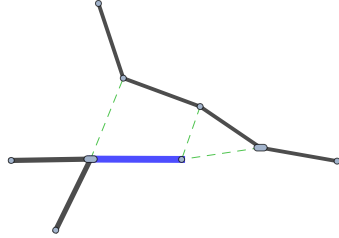
 $,$ 

$$\frac{G^3 m_2^2 \left( 6 \hat{n} \times \vec{S}_1 \cdot \vec{v}_2 \hat{n} \times \vec{S}_2 \cdot \vec{v}_2 + 2 \vec{S}_1 \cdot \vec{S}_2 (\hat{n} \cdot \vec{v}_2)^2 - 2 \hat{n} \cdot \vec{S}_1 \hat{n} \cdot \vec{v}_2 \vec{S}_2 \cdot \vec{v}_2 + 2 \vec{v}_2 \cdot \vec{v}_2 \hat{n} \cdot \vec{S}_1 \hat{n} \cdot \vec{S}_2 - 2 \vec{S}_1 \cdot \vec{S}_2 \vec{v}_2 \cdot \vec{v}_2 \right)}{r^5} \}$$

 $\{\text{DiagS1S2}[3, 2, 4],$ 
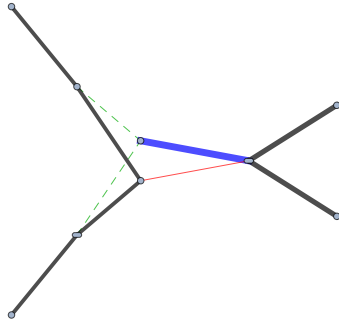
 $, \frac{1}{r^5}$ 

$$G^3 m_2^2 \left( -2 \hat{n} \times \vec{S}_1 \cdot \vec{v}_2 \hat{n} \times \vec{S}_2 \cdot \vec{v}_1 - 8 \hat{n} \times \vec{S}_1 \cdot \vec{v}_1 \hat{n} \times \vec{S}_2 \cdot \vec{v}_2 - 2 \vec{S}_1 \cdot \vec{S}_2 \hat{n} \cdot \vec{v}_1 \hat{n} \cdot \vec{v}_2 + 2 \hat{n} \cdot \vec{S}_1 \hat{n} \cdot \vec{v}_2 \vec{S}_2 \cdot \vec{v}_1 + 2 \vec{v}_1 \cdot \vec{v}_2 \hat{n} \cdot \vec{S}_1 \hat{n} \cdot \vec{S}_2 - 2 \vec{S}_1 \cdot \vec{S}_2 \vec{v}_1 \cdot \vec{v}_2 \right) \}$$

 $\{\text{DiagS1S2}[3, 2, 5],$ 
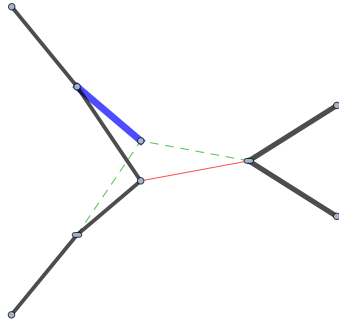
 $, \frac{1}{r^5}$ 

$$G^3 m_2^2 \left( -16 \hat{n} \times \vec{S}_1 \cdot \vec{v}_2 \hat{n} \times \vec{S}_2 \cdot \vec{v}_2 - 288 \hat{n} \cdot \vec{S}_1 \hat{n} \cdot \vec{S}_2 (\hat{n} \cdot \vec{v}_2)^2 + 32 \vec{S}_1 \cdot \vec{S}_2 (\hat{n} \cdot \vec{v}_2)^2 + 64 \hat{n} \cdot \vec{S}_2 \hat{n} \cdot \vec{v}_2 \vec{S}_1 \cdot \vec{v}_2 + 96 \hat{n} \cdot \vec{S}_1 \hat{n} \cdot \vec{v}_2 \vec{S}_2 \cdot \vec{v}_2 + 32 \vec{v}_2 \cdot \vec{v}_2 \hat{n} \cdot \vec{S}_1 \hat{n} \cdot \vec{S}_2 - 20 \vec{S}_1 \cdot \vec{v}_2 \vec{S}_2 \cdot \vec{v}_2 + 4 \vec{S}_1 \cdot \vec{S}_2 \vec{v}_2 \cdot \vec{v}_2 \right) \}$$

{DiagS1S2 [3, 2, 6],

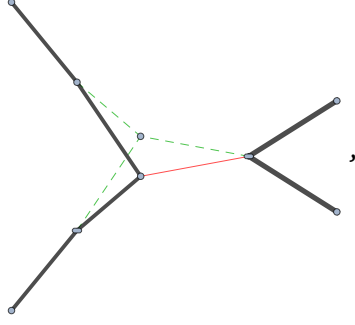

$$G^3 m_2^2 \left( \frac{1}{r^4} \left( 4 \vec{S}_1 \cdot \vec{a}_2 \hat{n} \cdot \vec{S}_2 - 4 \vec{S}_1 \cdot \vec{S}_2 \hat{n} \cdot \vec{a}_2 + 64 \hat{n} \cdot \vec{S}_2 \hat{n} \cdot \vec{S}_1 \hat{n} \cdot \vec{v}_2 - 48 \hat{n} \cdot \vec{S}_1 \hat{n} \cdot \vec{S}_2 \hat{n} \cdot \vec{v}_2 + 4 \vec{S}_1 \cdot \vec{S}_2 \hat{n} \cdot \vec{v}_2 + \right. \right. \\ \left. \left. 4 \vec{S}_1 \cdot \vec{S}_2 \hat{n} \cdot \vec{v}_2 + 8 \hat{n} \cdot \vec{S}_2 \vec{S}_1 \cdot \vec{v}_2 - 16 \hat{n} \cdot \vec{S}_1 \vec{S}_2 \cdot \vec{v}_2 - 20 \hat{n} \cdot \vec{S}_2 \vec{S}_1 \cdot \vec{v}_2 + 12 \hat{n} \cdot \vec{S}_1 \vec{S}_2 \cdot \vec{v}_2 \right) + \frac{1}{r^5} \right. \\ \left. \left( -32 \hat{n} \times \vec{S}_1 \cdot \vec{v}_2 \hat{n} \times \vec{S}_2 \cdot \vec{v}_2 + 240 \hat{n} \cdot \vec{S}_1 \hat{n} \cdot \vec{S}_2 (\hat{n} \cdot \vec{v}_2)^2 - 12 \vec{S}_1 \cdot \vec{S}_2 (\hat{n} \cdot \vec{v}_2)^2 + 336 \hat{n} \cdot \vec{S}_1 \hat{n} \cdot \vec{S}_2 \hat{n} \cdot \vec{v}_1 \hat{n} \cdot \vec{v}_2 - \right. \right. \\ \left. \left. 20 \vec{S}_1 \cdot \vec{S}_2 \hat{n} \cdot \vec{v}_1 \hat{n} \cdot \vec{v}_2 - 48 \hat{n} \cdot \vec{S}_2 \hat{n} \cdot \vec{v}_2 \vec{S}_1 \cdot \vec{v}_1 - 72 \hat{n} \cdot \vec{S}_2 \hat{n} \cdot \vec{v}_2 \vec{S}_1 \cdot \vec{v}_2 - 48 \hat{n} \cdot \vec{S}_1 \hat{n} \cdot \vec{v}_2 \vec{S}_2 \cdot \vec{v}_1 - \right. \right. \\ \left. \left. 84 \hat{n} \cdot \vec{S}_1 \hat{n} \cdot \vec{v}_2 \vec{S}_2 \cdot \vec{v}_2 - 40 \hat{n} \cdot \vec{S}_2 \hat{n} \cdot \vec{v}_1 \vec{S}_1 \cdot \vec{v}_2 - 60 \hat{n} \cdot \vec{S}_1 \hat{n} \cdot \vec{v}_1 \vec{S}_2 \cdot \vec{v}_2 - 48 \vec{v}_1 \cdot \vec{v}_2 \hat{n} \cdot \vec{S}_1 \hat{n} \cdot \vec{S}_2 - \right. \right. \\ \left. \left. 48 \vec{v}_2 \cdot \vec{v}_2 \hat{n} \cdot \vec{S}_1 \hat{n} \cdot \vec{S}_2 + 8 \vec{S}_1 \cdot \vec{v}_2 \vec{S}_2 \cdot \vec{v}_1 + 12 \vec{S}_1 \cdot \vec{v}_1 \vec{S}_2 \cdot \vec{v}_2 + 12 \vec{S}_1 \cdot \vec{v}_2 \vec{S}_2 \cdot \vec{v}_2 + 4 \vec{S}_1 \cdot \vec{S}_2 \vec{v}_1 \cdot \vec{v}_2 + 12 \vec{S}_1 \cdot \vec{S}_2 \vec{v}_2 \cdot \vec{v}_2 \right) \right) \Bigg\}$$

{DiagS1S2 [3, 2, 7],

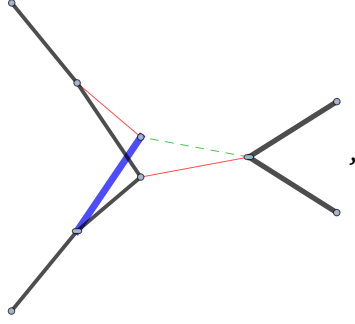

$$G^3 m_2^2 \left( \frac{1}{r^5} \left( -16 \hat{n} \times \vec{S}_1 \cdot \vec{v}_2 \hat{n} \times \vec{S}_2 \cdot \vec{v}_2 + 112 \hat{n} \cdot \vec{S}_1 \hat{n} \cdot \vec{S}_2 (\hat{n} \cdot \vec{v}_2)^2 + 20 \vec{S}_1 \cdot \vec{S}_2 (\hat{n} \cdot \vec{v}_2)^2 - 112 \hat{n} \cdot \vec{S}_1 \hat{n} \cdot \vec{S}_2 \hat{n} \cdot \vec{v}_1 \hat{n} \cdot \vec{v}_2 - \right. \right. \\ \left. \left. 20 \vec{S}_1 \cdot \vec{S}_2 \hat{n} \cdot \vec{v}_1 \hat{n} \cdot \vec{v}_2 + 16 \hat{n} \cdot \vec{S}_2 \hat{n} \cdot \vec{v}_2 \vec{S}_1 \cdot \vec{v}_1 - 56 \hat{n} \cdot \vec{S}_2 \hat{n} \cdot \vec{v}_2 \vec{S}_1 \cdot \vec{v}_2 + 16 \hat{n} \cdot \vec{S}_1 \hat{n} \cdot \vec{v}_2 \vec{S}_2 \cdot \vec{v}_1 - \right. \right. \\ \left. \left. 36 \hat{n} \cdot \vec{S}_1 \hat{n} \cdot \vec{v}_2 \vec{S}_2 \cdot \vec{v}_2 + 40 \hat{n} \cdot \vec{S}_2 \hat{n} \cdot \vec{v}_1 \vec{S}_1 \cdot \vec{v}_2 + 20 \hat{n} \cdot \vec{S}_1 \hat{n} \cdot \vec{v}_1 \vec{S}_2 \cdot \vec{v}_2 + 16 \vec{v}_1 \cdot \vec{v}_2 \hat{n} \cdot \vec{S}_1 \hat{n} \cdot \vec{S}_2 - \right. \right. \\ \left. \left. 16 \vec{v}_2 \cdot \vec{v}_2 \hat{n} \cdot \vec{S}_1 \hat{n} \cdot \vec{S}_2 - 8 \vec{S}_1 \cdot \vec{v}_2 \vec{S}_2 \cdot \vec{v}_1 - 4 \vec{S}_1 \cdot \vec{v}_1 \vec{S}_2 \cdot \vec{v}_2 + 8 \vec{S}_1 \cdot \vec{v}_2 \vec{S}_2 \cdot \vec{v}_2 + 4 \vec{S}_1 \cdot \vec{S}_2 \vec{v}_1 \cdot \vec{v}_2 \right) + \right. \\ \left. \frac{16 \hat{n} \cdot \vec{S}_1 \hat{n} \cdot \vec{S}_2 \hat{n} \cdot \vec{v}_2 + 4 \vec{S}_1 \cdot \vec{S}_2 \hat{n} \cdot \vec{v}_2 - 8 \hat{n} \cdot \vec{S}_2 \vec{S}_1 \cdot \vec{v}_2 - 4 \hat{n} \cdot \vec{S}_1 \vec{S}_2 \cdot \vec{v}_2}{r^4} \right) \Bigg\}$$

{DiagS1S2 [3, 2, 8],

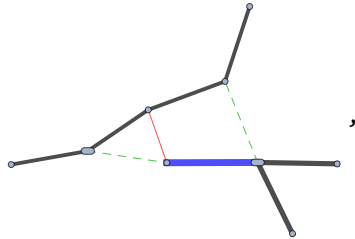

$$G^3 m_2^2 \left( \frac{-2 \hat{n} \times \vec{S}_1 \cdot \vec{v}_2 \hat{n} \times \vec{S}_2 \cdot \vec{v}_2 + 2 \vec{S}_1 \cdot \vec{S}_2 (\hat{n} \cdot \vec{v}_2)^2 - 2 \hat{n} \cdot \vec{S}_2 \hat{n} \cdot \vec{v}_2 \vec{S}_1 \cdot \vec{v}_2 + 2 \vec{S}_1 \cdot \vec{v}_2 \vec{S}_2 \cdot \vec{v}_2 - 2 \vec{S}_1 \cdot \vec{S}_2 \vec{v}_2 \cdot \vec{v}_2}{r^5} + \right.$$

$$\left. \frac{2 \hat{n} \cdot \vec{S}_1 \vec{S}_2 \cdot \vec{v}_2 - 2 \hat{n} \cdot \vec{S}_2 \hat{n} \cdot \vec{S}_1 \hat{n} \cdot \vec{v}_2}{r^4} \right\}$$

{DiagS1S2 [3, 2, 9],

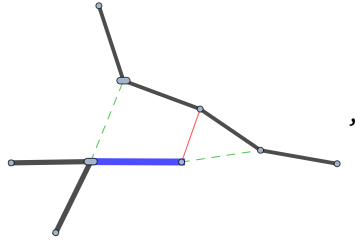

,

$$\left. \frac{G^3 m_2^2 \left( -12 \hat{n} \cdot \vec{a}_2 \hat{n} \cdot \vec{S}_1 \hat{n} \cdot \vec{S}_2 + 8 \vec{S}_1 \cdot \vec{a}_2 \hat{n} \cdot \vec{S}_2 + 8 \vec{S}_1 \cdot \vec{S}_2 \hat{n} \cdot \vec{a}_2 - 4 \vec{S}_2 \cdot \vec{a}_2 \hat{n} \cdot \vec{S}_1 \right)}{r^4} \right\}$$

{DiagS1S2 [3, 2, 10],

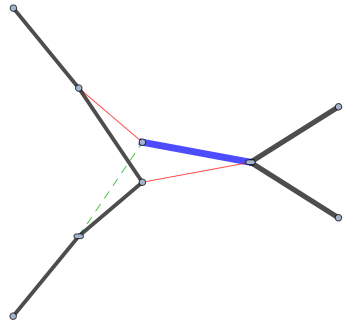

,

$$\left. \begin{aligned} & G^3 m_2^2 \left( \frac{2 \hat{n} \times \vec{S}_1 \cdot \vec{v}_1 \hat{n} \times \vec{S}_2 \cdot \vec{v}_2 + 2 \vec{S}_1 \cdot \vec{S}_2 \hat{n} \cdot \vec{v}_1 \hat{n} \cdot \vec{v}_2 - 2 \hat{n} \cdot \vec{S}_2 \hat{n} \cdot \vec{v}_1 \vec{S}_1 \cdot \vec{v}_2 - 2 \vec{S}_1 \cdot \vec{v}_2 \vec{S}_2 \cdot \vec{v}_1 + 2 \vec{S}_1 \cdot \vec{S}_2 \vec{v}_1 \cdot \vec{v}_2}{r^5} + \right. \\ & \left. \frac{-2 \hat{n} \cdot \vec{S}_2 \hat{n} \cdot \vec{S}_1 \hat{n} \cdot \vec{v}_1 + 4 \vec{S}_1 \cdot \vec{S}_2 \hat{n} \cdot \vec{v}_1 - 2 \hat{n} \cdot \vec{S}_1 \vec{S}_2 \cdot \vec{v}_1}{r^4} \right) \end{aligned} \right\}$$

{DiagS1S2 [3, 2, 11],

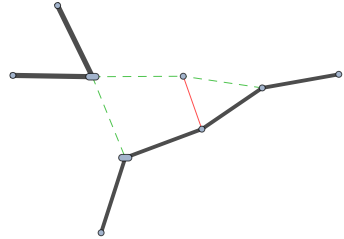

,  $G^3 m_2^2$

$$\left. \begin{aligned} & \left( \frac{-8 \vec{S}_1 \cdot \vec{S}_2 \hat{n} \cdot \vec{a}_2 + 8 \vec{S}_2 \cdot \vec{a}_2 \hat{n} \cdot \vec{S}_1 - 8 \hat{n} \cdot \vec{S}_1 \vec{S}_2 \cdot \vec{v}_2 + 8 \vec{S}_1 \cdot \vec{S}_2 \hat{n} \cdot \vec{v}_2}{r^4} + \frac{1}{r^5} \left( 16 \hat{n} \times \vec{S}_1 \cdot \vec{v}_2 \hat{n} \times \vec{S}_2 \cdot \vec{v}_1 + 8 \vec{S}_1 \cdot \vec{S}_2 (\hat{n} \cdot \vec{v}_2)^2 - \right. \right. \\ & \left. \left. 8 \hat{n} \cdot \vec{S}_1 \hat{n} \cdot \vec{v}_2 \vec{S}_2 \cdot \vec{v}_2 - 24 \vec{v}_1 \cdot \vec{v}_2 \hat{n} \cdot \vec{S}_1 \hat{n} \cdot \vec{S}_2 + 8 \vec{S}_1 \cdot \vec{v}_2 \vec{S}_2 \cdot \vec{v}_2 + 8 \vec{S}_1 \cdot \vec{S}_2 \vec{v}_1 \cdot \vec{v}_2 - 8 \vec{S}_1 \cdot \vec{S}_2 \vec{v}_2 \cdot \vec{v}_2 \right) \right) \end{aligned} \right\}$$

{DiagS1S2 [3, 2, 12],

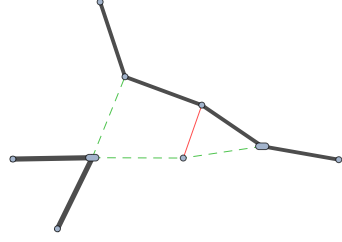

,  $G^3 m_2^2$

$$\left\{ \frac{-4 \vec{S}_1 \cdot \vec{S}_2 \hat{n} \cdot \vec{a}_2 + 4 \vec{S}_2 \cdot \vec{a}_2 \hat{n} \cdot \vec{S}_1 - 4 \hat{n} \cdot \vec{S}_1 \vec{S}_2 \cdot \vec{v}_2 + 4 \vec{S}_1 \cdot \vec{S}_2 \hat{n} \cdot \vec{v}_2}{r^4} + \frac{1}{r^5} \left( 4 \hat{n} \times \vec{S}_1 \cdot \vec{v}_2 \hat{n} \times \vec{S}_2 \cdot \vec{v}_1 + 12 \vec{S}_1 \cdot \vec{S}_2 (\hat{n} \cdot \vec{v}_2)^2 - \right. \right.$$

$$\left. \left. 12 \hat{n} \cdot \vec{S}_1 \hat{n} \cdot \vec{v}_2 \vec{S}_2 \cdot \vec{v}_2 - 16 \vec{v}_1 \cdot \vec{v}_2 \hat{n} \cdot \vec{S}_1 \hat{n} \cdot \vec{S}_2 + 4 \vec{S}_1 \cdot \vec{v}_2 \vec{S}_2 \cdot \vec{v}_2 + 8 \vec{S}_1 \cdot \vec{S}_2 \vec{v}_1 \cdot \vec{v}_2 - 4 \vec{S}_1 \cdot \vec{S}_2 \vec{v}_2 \cdot \vec{v}_2 \right) \right\}$$

{DiagS1S2 [3, 2, 13],

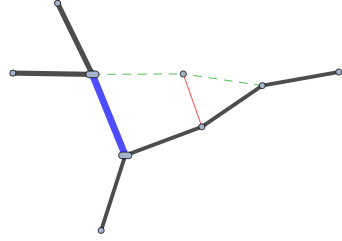

,

$$\frac{G^3 m_2^2 \left( 24 \hat{n} \times \vec{S}_1 \cdot \vec{v}_2 \hat{n} \times \vec{S}_2 \cdot \vec{v}_2 + 8 \vec{S}_1 \cdot \vec{S}_2 (\hat{n} \cdot \vec{v}_2)^2 - 8 \hat{n} \cdot \vec{S}_1 \hat{n} \cdot \vec{v}_2 \vec{S}_2 \cdot \vec{v}_2 + 8 \vec{v}_2 \cdot \vec{v}_2 \hat{n} \cdot \vec{S}_1 \hat{n} \cdot \vec{S}_2 - 8 \vec{S}_1 \cdot \vec{S}_2 \vec{v}_2 \cdot \vec{v}_2 \right)}{r^5} \Bigg\}$$

{DiagS1S2 [3, 2, 14],

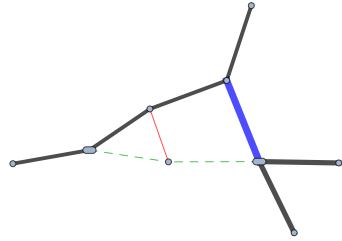

,  $\frac{1}{r^5}$

$$G^3 m_2^2 \left( -8 \hat{n} \times \vec{S}_1 \cdot \vec{v}_2 \hat{n} \times \vec{S}_2 \cdot \vec{v}_2 - 8 \vec{S}_1 \cdot \vec{S}_2 (\hat{n} \cdot \vec{v}_2)^2 + 8 \hat{n} \cdot \vec{S}_1 \hat{n} \cdot \vec{v}_2 \vec{S}_2 \cdot \vec{v}_2 - \right.$$

$$\left. 16 \vec{v}_2 \cdot \vec{v}_2 \hat{n} \cdot \vec{S}_1 \hat{n} \cdot \vec{S}_2 - 4 \vec{S}_1 \cdot \vec{v}_2 \vec{S}_2 \cdot \vec{v}_2 + 12 \vec{S}_1 \cdot \vec{S}_2 \vec{v}_2 \cdot \vec{v}_2 \right) \Bigg\}$$

{DiagS1S2 [3, 2, 15],

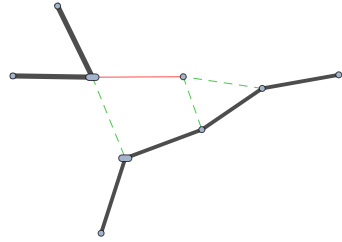

$$, \frac{G^3 m_2^2 \left( 48 \vec{v}_2 \cdot \vec{v}_2 \hat{n} \cdot \vec{S}_1 \hat{n} \cdot \vec{S}_2 - 16 \vec{S}_1 \cdot \vec{S}_2 \vec{v}_2 \cdot \vec{v}_2 \right)}{r^5} \Bigg\}$$

{DiagS1S2 [3, 2, 16],

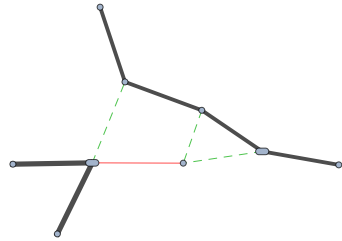

$$, - \frac{16 G^3 m_2^2 \hat{n} \times \vec{S}_1 \cdot \vec{v}_2 \hat{n} \times \vec{S}_2 \cdot \vec{v}_2}{r^5} \Bigg\}$$

$\{\text{DiagS1S2}[3, 2, 17],$ 
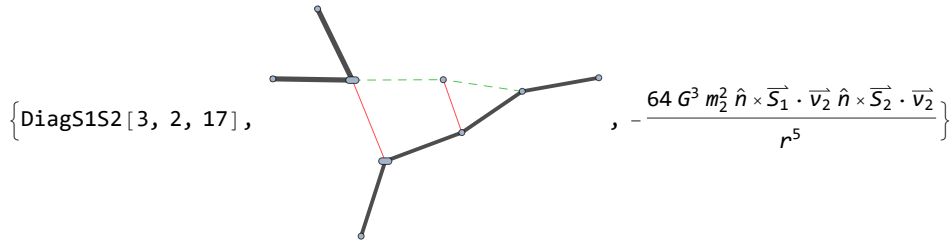
 $, -\frac{64 G^3 m_2^2 \hat{n} \times \vec{S}_1 \cdot \vec{v}_2 \hat{n} \times \vec{S}_2 \cdot \vec{v}_2}{r^5} \}$

$\{\text{DiagS1S2}[3, 2, 18],$ 
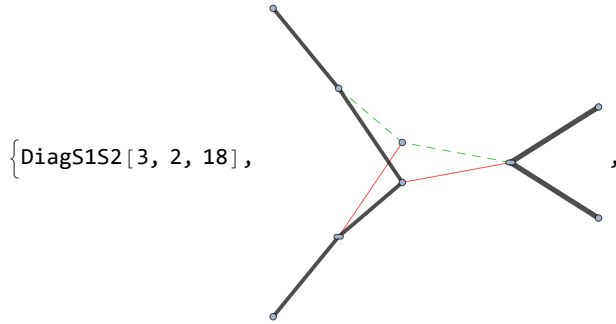
 $,$

$$\frac{G^3 m_2^2 \left( -128 \hat{n} \times \vec{S}_1 \cdot \vec{v}_2 \hat{n} \times \vec{S}_2 \cdot \vec{v}_2 - 64 \vec{S}_1 \cdot \vec{S}_2 (\hat{n} \cdot \vec{v}_2)^2 + 64 \hat{n} \cdot \vec{S}_2 \hat{n} \cdot \vec{v}_2 \vec{S}_1 \cdot \vec{v}_2 - 48 \vec{S}_1 \cdot \vec{v}_2 \vec{S}_2 \cdot \vec{v}_2 + 48 \vec{S}_1 \cdot \vec{S}_2 \vec{v}_2 \cdot \vec{v}_2 \right)}{r^5} \}$$

$\{\text{DiagS1S2}[3, 2, 19],$ 
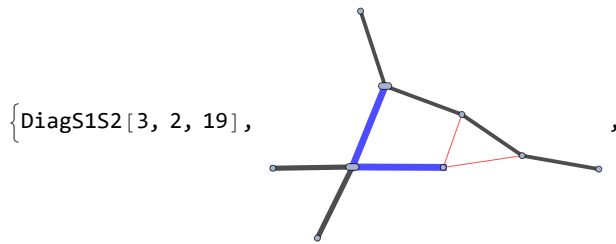
 $,$

$$G^3 m_2^2 \left( \frac{-\frac{1}{4} \hat{n} \cdot \vec{a}_2 \hat{n} \cdot \vec{S}_1 \hat{n} \cdot \vec{S}_2 + \frac{1}{4} \vec{S}_1 \cdot \vec{S}_2 \hat{n} \cdot \vec{a}_2 - \frac{1}{4} \hat{n} \cdot \vec{S}_2 \hat{n} \cdot \vec{S}_1 \hat{n} \cdot \vec{v}_2 + \frac{1}{4} \vec{S}_1 \cdot \vec{S}_2 \hat{n} \cdot \vec{v}_2}{r^4} + \frac{1}{r^5} \right. \\ \left. \left( -3 \hat{n} \times \vec{S}_1 \cdot \vec{v}_2 \hat{n} \times \vec{S}_2 \cdot \vec{v}_1 + 6 \hat{n} \times \vec{S}_1 \cdot \vec{v}_1 \hat{n} \times \vec{S}_2 \cdot \vec{v}_2 + \frac{1}{2} \hat{n} \times \vec{S}_1 \cdot \vec{v}_2 \hat{n} \times \vec{S}_2 \cdot \vec{v}_2 + \frac{1}{4} \hat{n} \cdot \vec{S}_1 \hat{n} \cdot \vec{S}_2 (\hat{n} \cdot \vec{v}_2)^2 - \right. \right. \\ \left. \frac{1}{4} \vec{S}_1 \cdot \vec{S}_2 (\hat{n} \cdot \vec{v}_2)^2 - \frac{1}{4} \hat{n} \cdot \vec{S}_1 \hat{n} \cdot \vec{S}_2 \hat{n} \cdot \vec{v}_1 \hat{n} \cdot \vec{v}_2 + \frac{5}{4} \vec{S}_1 \cdot \vec{S}_2 \hat{n} \cdot \vec{v}_1 \hat{n} \cdot \vec{v}_2 + \frac{1}{4} \hat{n} \cdot \vec{S}_2 \hat{n} \cdot \vec{v}_2 \vec{S}_1 \cdot \vec{v}_1 + \right. \\ \left. \frac{1}{4} \hat{n} \cdot \vec{S}_2 \hat{n} \cdot \vec{v}_2 \vec{S}_1 \cdot \vec{v}_2 - \frac{1}{4} \hat{n} \cdot \vec{S}_1 \hat{n} \cdot \vec{v}_2 \vec{S}_2 \cdot \vec{v}_1 - \frac{1}{4} \hat{n} \cdot \vec{S}_1 \hat{n} \cdot \vec{v}_2 \vec{S}_2 \cdot \vec{v}_2 - \hat{n} \cdot \vec{S}_2 \hat{n} \cdot \vec{v}_1 \vec{S}_1 \cdot \vec{v}_2 + \frac{13}{4} \vec{v}_1 \cdot \vec{v}_2 \hat{n} \cdot \vec{S}_1 \hat{n} \cdot \vec{S}_2 - \right. \\ \left. \left. \frac{1}{4} \vec{v}_2 \cdot \vec{v}_2 \hat{n} \cdot \vec{S}_1 \hat{n} \cdot \vec{S}_2 + 2 \vec{S}_1 \cdot \vec{v}_2 \vec{S}_2 \cdot \vec{v}_1 - \vec{S}_1 \cdot \vec{v}_1 \vec{S}_2 \cdot \vec{v}_2 - \frac{9}{4} \vec{S}_1 \cdot \vec{S}_2 \vec{v}_1 \cdot \vec{v}_2 + \frac{1}{4} \vec{S}_1 \cdot \vec{S}_2 \vec{v}_2 \cdot \vec{v}_2 \right) \right) \}$$

$\{\text{DiagS1S2}[3, 2, 20],$ 
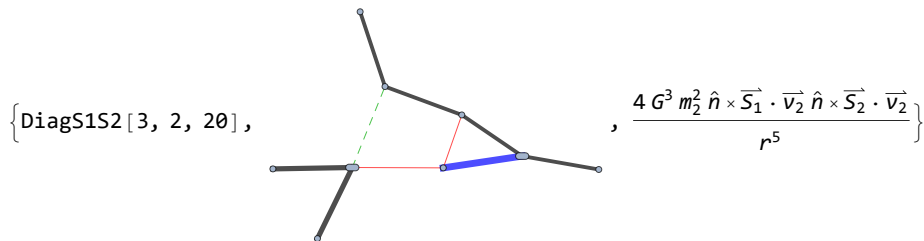
 $, \frac{4 G^3 m_2^2 \hat{n} \times \vec{S}_1 \cdot \vec{v}_2 \hat{n} \times \vec{S}_2 \cdot \vec{v}_2}{r^5} \}$



{DiagS1S2 [3, 2, 21],

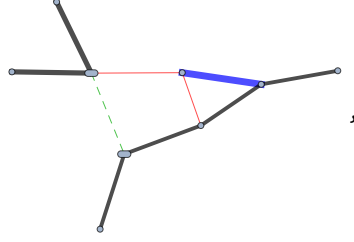

$$\frac{G^3 m_2^2 \left( -48 \hat{n} \cdot \vec{S}_1 \hat{n} \cdot \vec{S}_2 (\hat{n} \cdot \vec{v}_2)^2 + 16 \vec{S}_1 \cdot \vec{S}_2 (\hat{n} \cdot \vec{v}_2)^2 + 24 \vec{v}_2 \cdot \vec{v}_2 \hat{n} \cdot \vec{S}_1 \hat{n} \cdot \vec{S}_2 - 8 \vec{S}_1 \cdot \vec{S}_2 \vec{v}_2 \cdot \vec{v}_2 \right)}{r^5} \}$$

{DiagS1S2 [3, 2, 22],

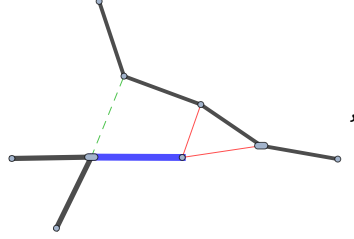

$$\frac{G^3 m_2^2 \left( 2 \hat{n} \times \vec{S}_1 \cdot \vec{v}_2 \hat{n} \times \vec{S}_2 \cdot \vec{v}_2 - 2 \vec{S}_1 \cdot \vec{S}_2 (\hat{n} \cdot \vec{v}_2)^2 + 2 \hat{n} \cdot \vec{S}_2 \hat{n} \cdot \vec{v}_2 \vec{S}_1 \cdot \vec{v}_2 - 2 \vec{S}_1 \cdot \vec{v}_2 \vec{S}_2 \cdot \vec{v}_2 + 2 \vec{S}_1 \cdot \vec{S}_2 \vec{v}_2 \cdot \vec{v}_2 \right)}{r^5} \}$$

{DiagS1S2 [3, 2, 23],

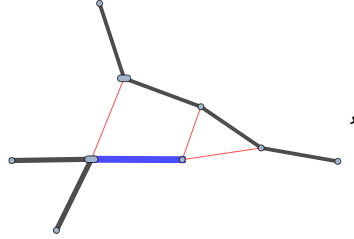

$$\frac{G^3 m_2^2 \left( 4 \hat{n} \times \vec{S}_1 \cdot \vec{v}_1 \hat{n} \times \vec{S}_2 \cdot \vec{v}_2 + 2 \vec{S}_1 \cdot \vec{S}_2 \hat{n} \cdot \vec{v}_1 \hat{n} \cdot \vec{v}_2 - 2 \hat{n} \cdot \vec{S}_2 \hat{n} \cdot \vec{v}_1 \vec{S}_1 \cdot \vec{v}_2 \right)}{r^5} \}$$

{DiagS1S2 [3, 2, 24],

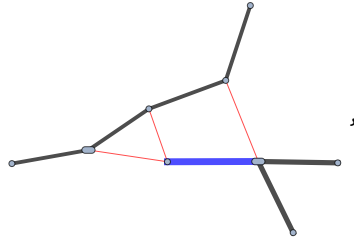

$$\frac{G^3 m_2^2 \left( 6 \hat{n} \times \vec{S}_1 \cdot \vec{v}_1 \hat{n} \times \vec{S}_2 \cdot \vec{v}_2 - 2 \vec{S}_1 \cdot \vec{S}_2 \hat{n} \cdot \vec{v}_1 \hat{n} \cdot \vec{v}_2 + 2 \hat{n} \cdot \vec{S}_2 \hat{n} \cdot \vec{v}_1 \vec{S}_1 \cdot \vec{v}_2 + 2 \vec{S}_1 \cdot \vec{v}_2 \vec{S}_2 \cdot \vec{v}_1 - 2 \vec{S}_1 \cdot \vec{S}_2 \vec{v}_1 \cdot \vec{v}_2 \right)}{r^5} \}$$

{DiagS1S2 [3, 2, 25],

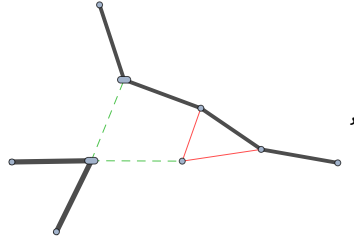

$$G^3 m_2^2 \left\{ \frac{\hat{n} \cdot \vec{a}_2 \hat{n} \cdot \vec{S}_1 \hat{n} \cdot \vec{S}_2 - \vec{S}_2 \cdot \vec{a}_2 \hat{n} \cdot \vec{S}_1 - \hat{n} \cdot \vec{S}_2 \hat{n} \cdot \vec{S}_1 \hat{n} \cdot \vec{v}_2 + \hat{n} \cdot \vec{S}_1 \vec{S}_2 \cdot \vec{v}_2}{r^4} + \frac{1}{r^5} \right. \\ \left. \left( -\hat{n} \times \vec{S}_1 \cdot \vec{v}_2 \hat{n} \times \vec{S}_2 \cdot \vec{v}_1 + \hat{n} \cdot \vec{S}_1 \hat{n} \cdot \vec{S}_2 (\hat{n} \cdot \vec{v}_2)^2 - 2 \vec{S}_1 \cdot \vec{S}_2 (\hat{n} \cdot \vec{v}_2)^2 - 3 \hat{n} \cdot \vec{S}_1 \hat{n} \cdot \vec{S}_2 \hat{n} \cdot \vec{v}_1 \hat{n} \cdot \vec{v}_2 + \vec{S}_1 \cdot \vec{S}_2 \hat{n} \cdot \vec{v}_1 \hat{n} \cdot \vec{v}_2 + \right. \right. \\ \left. \left. \hat{n} \cdot \vec{S}_2 \hat{n} \cdot \vec{v}_2 \vec{S}_1 \cdot \vec{v}_2 + 3 \vec{v}_1 \cdot \vec{v}_2 \hat{n} \cdot \vec{S}_1 \hat{n} \cdot \vec{S}_2 - \vec{v}_2 \cdot \vec{v}_2 \hat{n} \cdot \vec{S}_1 \hat{n} \cdot \vec{S}_2 - \vec{S}_1 \cdot \vec{v}_2 \vec{S}_2 \cdot \vec{v}_2 - \vec{S}_1 \cdot \vec{S}_2 \vec{v}_1 \cdot \vec{v}_2 + 2 \vec{S}_1 \cdot \vec{S}_2 \vec{v}_2 \cdot \vec{v}_2 \right) \right\}$$

{DiagS1S2 [3, 2, 26],

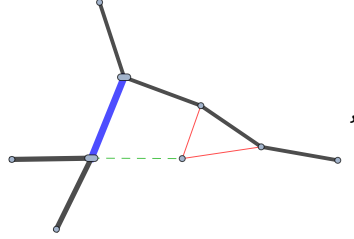

$$\frac{G^3 m_2^2 \left( -\frac{3}{2} \hat{n} \times \vec{S}_1 \cdot \vec{v}_2 \hat{n} \times \vec{S}_2 \cdot \vec{v}_2 - \frac{1}{2} \vec{S}_1 \cdot \vec{S}_2 (\hat{n} \cdot \vec{v}_2)^2 + \frac{1}{2} \hat{n} \cdot \vec{S}_1 \hat{n} \cdot \vec{v}_2 \vec{S}_2 \cdot \vec{v}_2 - \frac{1}{2} \vec{v}_2 \cdot \vec{v}_2 \hat{n} \cdot \vec{S}_1 \hat{n} \cdot \vec{S}_2 + \frac{1}{2} \vec{S}_1 \cdot \vec{S}_2 \vec{v}_2 \cdot \vec{v}_2 \right)}{r^5} \}$$

{DiagS1S2 [3, 2, 27],

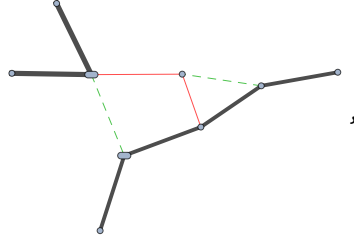

$$G^3 m_2^2 \left\{ \frac{1}{r^5} \left( -72 \hat{n} \cdot \vec{S}_1 \hat{n} \cdot \vec{S}_2 (\hat{n} \cdot \vec{v}_2)^2 + 8 \vec{S}_1 \cdot \vec{S}_2 (\hat{n} \cdot \vec{v}_2)^2 + 168 \hat{n} \cdot \vec{S}_1 \hat{n} \cdot \vec{S}_2 \hat{n} \cdot \vec{v}_1 \hat{n} \cdot \vec{v}_2 - \right. \right. \\ \left. \left. 40 \vec{S}_1 \cdot \vec{S}_2 \hat{n} \cdot \vec{v}_1 \hat{n} \cdot \vec{v}_2 - 24 \hat{n} \cdot \vec{S}_2 \hat{n} \cdot \vec{v}_2 \vec{S}_1 \cdot \vec{v}_1 + 24 \hat{n} \cdot \vec{S}_2 \hat{n} \cdot \vec{v}_2 \vec{S}_1 \cdot \vec{v}_2 - 24 \hat{n} \cdot \vec{S}_1 \hat{n} \cdot \vec{v}_2 \vec{S}_2 \cdot \vec{v}_1 + \right. \right. \\ \left. \left. 24 \hat{n} \cdot \vec{S}_1 \hat{n} \cdot \vec{v}_2 \vec{S}_2 \cdot \vec{v}_2 - 24 \vec{v}_1 \cdot \vec{v}_2 \hat{n} \cdot \vec{S}_1 \hat{n} \cdot \vec{S}_2 - 24 \vec{v}_2 \cdot \vec{v}_2 \hat{n} \cdot \vec{S}_1 \hat{n} \cdot \vec{S}_2 + 8 \vec{S}_1 \cdot \vec{S}_2 \vec{v}_1 \cdot \vec{v}_2 + 8 \vec{S}_1 \cdot \vec{S}_2 \vec{v}_2 \cdot \vec{v}_2 \right) + \right. \\ \left. \frac{-24 \hat{n} \cdot \vec{S}_2 \hat{n} \cdot \vec{S}_1 \hat{n} \cdot \vec{v}_2 - 24 \hat{n} \cdot \vec{S}_1 \hat{n} \cdot \vec{S}_2 \hat{n} \cdot \vec{v}_2 + 8 \vec{S}_1 \cdot \vec{S}_2 \hat{n} \cdot \vec{v}_2 + 8 \vec{S}_1 \cdot \vec{S}_2 \hat{n} \cdot \vec{v}_2}{r^4} \right\}$$

{DiagS1S2 [3, 2, 28],

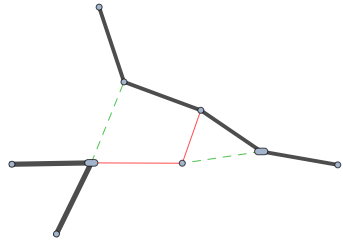

$$, - \frac{4 G^3 m_2^2 \hat{n} \times \vec{S}_1 \cdot \vec{v}_2 \hat{n} \times \vec{S}_2 \cdot \vec{v}_2}{r^5} \}$$

{DiagS1S2 [3, 2, 29],

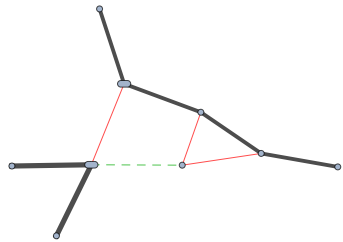

$$, \frac{4 G^3 m_2^2 \hat{n} \times \vec{S}_1 \cdot \vec{v}_2 \hat{n} \times \vec{S}_2 \cdot \vec{v}_2}{r^5} \}$$

{DiagS1S2 [3, 2, 30],

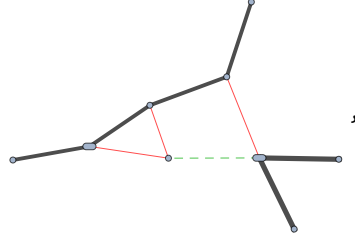

$$G^3 m_2^2 \left( \frac{4 \vec{S}_1 \cdot \vec{a}_2 \hat{n} \cdot \vec{S}_2 - 4 \vec{S}_1 \cdot \vec{S}_2 \hat{n} \cdot \vec{a}_2 - 4 \vec{S}_1 \cdot \vec{S}_2 \hat{n} \cdot \vec{v}_2 + 4 \hat{n} \cdot \vec{S}_2 \vec{S}_1 \cdot \vec{v}_2}{r^4} + \right. \\ \left. \frac{16 \hat{n} \times \vec{S}_1 \cdot \vec{v}_2 \hat{n} \times \vec{S}_2 \cdot \vec{v}_2 + 4 \vec{S}_1 \cdot \vec{v}_2 \vec{S}_2 \cdot \vec{v}_2 - 4 \vec{S}_1 \cdot \vec{S}_2 \vec{v}_2 \cdot \vec{v}_2}{r^5} \right\}$$

{DiagS1S2 [3, 2, 31],

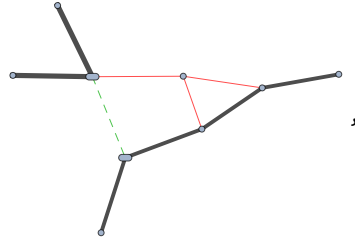

$$G^3 m_2^2 \left( \frac{1}{r^5} \left( 126 \hat{n} \cdot \vec{S}_1 \hat{n} \cdot \vec{S}_2 (\hat{n} \cdot \vec{v}_2)^2 - 26 \vec{S}_1 \cdot \vec{S}_2 (\hat{n} \cdot \vec{v}_2)^2 - 168 \hat{n} \cdot \vec{S}_1 \hat{n} \cdot \vec{S}_2 \hat{n} \cdot \vec{v}_1 \hat{n} \cdot \vec{v}_2 + \right. \right. \\ 40 \vec{S}_1 \cdot \vec{S}_2 \hat{n} \cdot \vec{v}_1 \hat{n} \cdot \vec{v}_2 + 24 \hat{n} \cdot \vec{S}_2 \hat{n} \cdot \vec{v}_2 \vec{S}_1 \cdot \vec{v}_1 - 24 \hat{n} \cdot \vec{S}_2 \hat{n} \cdot \vec{v}_2 \vec{S}_1 \cdot \vec{v}_2 + 24 \hat{n} \cdot \vec{S}_1 \hat{n} \cdot \vec{v}_2 \vec{S}_2 \cdot \vec{v}_1 - \\ 24 \hat{n} \cdot \vec{S}_1 \hat{n} \cdot \vec{v}_2 \vec{S}_2 \cdot \vec{v}_2 + 24 \vec{v}_1 \cdot \vec{v}_2 \hat{n} \cdot \vec{S}_1 \hat{n} \cdot \vec{S}_2 - 6 \vec{v}_2 \cdot \vec{v}_2 \hat{n} \cdot \vec{S}_1 \hat{n} \cdot \vec{S}_2 - 8 \vec{S}_1 \cdot \vec{S}_2 \vec{v}_1 \cdot \vec{v}_2 + 2 \vec{S}_1 \cdot \vec{S}_2 \vec{v}_2 \cdot \vec{v}_2 \Big) + \\ \left. \frac{24 \hat{n} \cdot \vec{S}_2 \hat{n} \cdot \vec{S}_1 \hat{n} \cdot \vec{v}_2 + 24 \hat{n} \cdot \vec{S}_1 \hat{n} \cdot \vec{S}_2 \hat{n} \cdot \vec{v}_2 - 8 \vec{S}_1 \cdot \vec{S}_2 \hat{n} \cdot \vec{v}_2 - 8 \vec{S}_1 \cdot \vec{S}_2 \hat{n} \cdot \vec{v}_2}{r^4} \right\}$$

{DiagS1S2 [3, 2, 32],

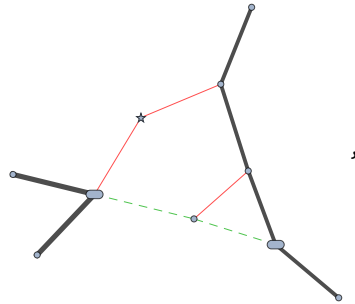

$$G^3 m_2^2 \left( \frac{1}{r^5} \left( 48 \hat{n} \cdot \vec{S}_1 \hat{n} \cdot \vec{S}_2 (\hat{n} \cdot \vec{v}_2)^2 - 16 \vec{S}_1 \cdot \vec{S}_2 (\hat{n} \cdot \vec{v}_2)^2 - 56 \hat{n} \cdot \vec{S}_1 \hat{n} \cdot \vec{S}_2 \hat{n} \cdot \vec{v}_1 \hat{n} \cdot \vec{v}_2 + 20 \vec{S}_1 \cdot \vec{S}_2 \hat{n} \cdot \vec{v}_1 \hat{n} \cdot \vec{v}_2 + \right. \right. \\ 8 \hat{n} \cdot \vec{S}_2 \hat{n} \cdot \vec{v}_2 \vec{S}_1 \cdot \vec{v}_1 - 8 \hat{n} \cdot \vec{S}_2 \hat{n} \cdot \vec{v}_2 \vec{S}_1 \cdot \vec{v}_2 + 8 \hat{n} \cdot \vec{S}_1 \hat{n} \cdot \vec{v}_2 \vec{S}_2 \cdot \vec{v}_1 - 8 \hat{n} \cdot \vec{S}_1 \hat{n} \cdot \vec{v}_2 \vec{S}_2 \cdot \vec{v}_2 + 8 \vec{v}_1 \cdot \vec{v}_2 \hat{n} \cdot \vec{S}_1 \hat{n} \cdot \vec{S}_2 - \\ 4 \vec{S}_1 \cdot \vec{S}_2 \vec{v}_1 \cdot \vec{v}_2 \Big) + \frac{8 \hat{n} \cdot \vec{S}_2 \hat{n} \cdot \vec{S}_1 \hat{n} \cdot \vec{v}_2 + 8 \hat{n} \cdot \vec{S}_1 \hat{n} \cdot \vec{S}_2 \hat{n} \cdot \vec{v}_2 - 4 \vec{S}_1 \cdot \vec{S}_2 \hat{n} \cdot \vec{v}_2 - 4 \vec{S}_1 \cdot \vec{S}_2 \hat{n} \cdot \vec{v}_2}{r^4} \Big) \Big\}$$

{DiagS1S2 [3, 2, 33],

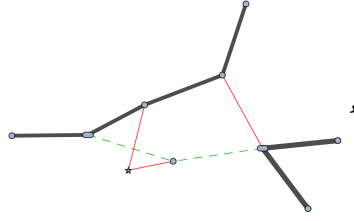

,

$$G^3 m_2^2 \left( \frac{1}{r^5} \left( 8 \hat{n} \times \vec{S}_1 \cdot \vec{v}_2 \hat{n} \times \vec{S}_2 \cdot \vec{v}_2 + 88 \hat{n} \cdot \vec{S}_1 \hat{n} \cdot \vec{S}_2 (\hat{n} \cdot \vec{v}_2)^2 - 14 \vec{S}_1 \cdot \vec{S}_2 (\hat{n} \cdot \vec{v}_2)^2 - 112 \hat{n} \cdot \vec{S}_1 \hat{n} \cdot \vec{S}_2 \hat{n} \cdot \vec{v}_1 \hat{n} \cdot \vec{v}_2 + \right. \right. \\ \left. \left. 30 \vec{S}_1 \cdot \vec{S}_2 \hat{n} \cdot \vec{v}_1 \hat{n} \cdot \vec{v}_2 + 16 \hat{n} \cdot \vec{S}_2 \hat{n} \cdot \vec{v}_2 \vec{S}_1 \cdot \vec{v}_1 - 14 \hat{n} \cdot \vec{S}_2 \hat{n} \cdot \vec{v}_2 \vec{S}_1 \cdot \vec{v}_2 + 16 \hat{n} \cdot \vec{S}_1 \hat{n} \cdot \vec{v}_2 \vec{S}_2 \cdot \vec{v}_1 - \right. \right. \\ \left. \left. 28 \hat{n} \cdot \vec{S}_1 \hat{n} \cdot \vec{v}_2 \vec{S}_2 \cdot \vec{v}_2 - 10 \hat{n} \cdot \vec{S}_2 \hat{n} \cdot \vec{v}_1 \vec{S}_1 \cdot \vec{v}_2 + 20 \hat{n} \cdot \vec{S}_1 \hat{n} \cdot \vec{v}_1 \vec{S}_2 \cdot \vec{v}_2 + 16 \vec{v}_1 \cdot \vec{v}_2 \hat{n} \cdot \vec{S}_1 \hat{n} \cdot \vec{S}_2 + \right. \right. \\ \left. \left. 2 \vec{S}_1 \cdot \vec{v}_2 \vec{S}_2 \cdot \vec{v}_1 - 4 \vec{S}_1 \cdot \vec{v}_1 \vec{S}_2 \cdot \vec{v}_2 + 6 \vec{S}_1 \cdot \vec{v}_2 \vec{S}_2 \cdot \vec{v}_2 - 6 \vec{S}_1 \cdot \vec{S}_2 \vec{v}_1 \cdot \vec{v}_2 - 6 \vec{S}_1 \cdot \vec{S}_2 \vec{v}_2 \cdot \vec{v}_2 \right) + \right. \\ \left. \frac{1}{r^4} \left( 16 \hat{n} \cdot \vec{S}_2 \hat{n} \cdot \vec{S}_1 \hat{n} \cdot \vec{v}_2 + 16 \hat{n} \cdot \vec{S}_1 \hat{n} \cdot \vec{S}_2 \hat{n} \cdot \vec{v}_2 - 6 \vec{S}_1 \cdot \vec{S}_2 \hat{n} \cdot \vec{v}_2 - 6 \vec{S}_1 \cdot \vec{S}_2 \hat{n} \cdot \vec{v}_2 + \right. \right. \\ \left. \left. 2 \hat{n} \cdot \vec{S}_2 \vec{S}_1 \cdot \vec{v}_2 - 4 \hat{n} \cdot \vec{S}_1 \vec{S}_2 \cdot \vec{v}_2 + 2 \hat{n} \cdot \vec{S}_2 \vec{S}_1 \cdot \vec{v}_2 - 4 \hat{n} \cdot \vec{S}_1 \vec{S}_2 \cdot \vec{v}_2 \right) \right) \Bigg\}$$

{DiagS1S2 [3, 2, 34],

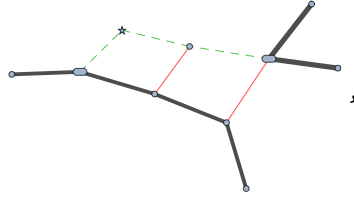

,

$$G^3 m_2^2 \left( \frac{1}{r^5} \left( 8 \hat{n} \times \vec{S}_1 \cdot \vec{v}_2 \hat{n} \times \vec{S}_2 \cdot \vec{v}_2 + 120 \hat{n} \cdot \vec{S}_1 \hat{n} \cdot \vec{S}_2 (\hat{n} \cdot \vec{v}_2)^2 + 10 \vec{S}_1 \cdot \vec{S}_2 (\hat{n} \cdot \vec{v}_2)^2 - 336 \hat{n} \cdot \vec{S}_1 \hat{n} \cdot \vec{S}_2 \hat{n} \cdot \vec{v}_1 \hat{n} \cdot \vec{v}_2 - \right. \right. \\ \left. \left. 10 \vec{S}_1 \cdot \vec{S}_2 \hat{n} \cdot \vec{v}_1 \hat{n} \cdot \vec{v}_2 + 48 \hat{n} \cdot \vec{S}_2 \hat{n} \cdot \vec{v}_2 \vec{S}_1 \cdot \vec{v}_1 - 46 \hat{n} \cdot \vec{S}_2 \hat{n} \cdot \vec{v}_2 \vec{S}_1 \cdot \vec{v}_2 + 48 \hat{n} \cdot \vec{S}_1 \hat{n} \cdot \vec{v}_2 \vec{S}_2 \cdot \vec{v}_1 - \right. \right. \\ \left. \left. 36 \hat{n} \cdot \vec{S}_1 \hat{n} \cdot \vec{v}_2 \vec{S}_2 \cdot \vec{v}_2 + 70 \hat{n} \cdot \vec{S}_2 \hat{n} \cdot \vec{v}_1 \vec{S}_1 \cdot \vec{v}_2 + 60 \hat{n} \cdot \vec{S}_1 \hat{n} \cdot \vec{v}_1 \vec{S}_2 \cdot \vec{v}_2 + 48 \vec{v}_1 \cdot \vec{v}_2 \hat{n} \cdot \vec{S}_1 \hat{n} \cdot \vec{S}_2 - \right. \right. \\ \left. \left. 16 \vec{v}_2 \cdot \vec{v}_2 \hat{n} \cdot \vec{S}_1 \hat{n} \cdot \vec{S}_2 - 14 \vec{S}_1 \cdot \vec{v}_2 \vec{S}_2 \cdot \vec{v}_1 - 12 \vec{S}_1 \cdot \vec{v}_1 \vec{S}_2 \cdot \vec{v}_2 + 10 \vec{S}_1 \cdot \vec{v}_2 \vec{S}_2 \cdot \vec{v}_2 + 2 \vec{S}_1 \cdot \vec{S}_2 \vec{v}_1 \cdot \vec{v}_2 - 2 \vec{S}_1 \cdot \vec{S}_2 \vec{v}_2 \cdot \vec{v}_2 \right) + \right. \\ \left. \frac{1}{r^4} \left( -120 \hat{n} \cdot \vec{S}_2 \hat{n} \cdot \vec{S}_1 \hat{n} \cdot \vec{v}_1 + 72 \hat{n} \cdot \vec{S}_2 \hat{n} \cdot \vec{S}_1 \hat{n} \cdot \vec{v}_2 + 48 \hat{n} \cdot \vec{S}_1 \hat{n} \cdot \vec{S}_2 \hat{n} \cdot \vec{v}_2 + 2 \vec{S}_1 \cdot \vec{S}_2 \hat{n} \cdot \vec{v}_2 - \right. \right. \\ \left. \left. 14 \hat{n} \cdot \vec{S}_2 \vec{S}_1 \cdot \vec{v}_2 + 24 \hat{n} \cdot \vec{S}_1 \vec{S}_2 \cdot \vec{v}_1 - 12 \hat{n} \cdot \vec{S}_1 \vec{S}_2 \cdot \vec{v}_2 - 2 \vec{S}_1 \cdot \vec{S}_2 \hat{n} \cdot \vec{v}_2 + \right. \right. \\ \left. \left. 24 \hat{n} \cdot \vec{S}_2 \vec{S}_1 \cdot \vec{v}_1 - 10 \hat{n} \cdot \vec{S}_2 \vec{S}_1 \cdot \vec{v}_2 - 12 \hat{n} \cdot \vec{S}_1 \vec{S}_2 \cdot \vec{v}_2 \right) + \frac{24 \hat{n} \cdot \vec{S}_1 \hat{n} \cdot \vec{S}_2}{r^3} \right) \Bigg\}$$

{DiagS1S2 [3, 2, 35],

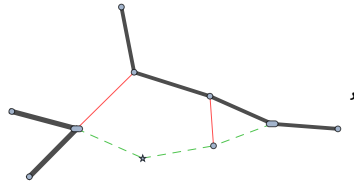

,

$$G^3 m_2^2 \left( \frac{1}{r^5} \left( 16 \hat{n} \cdot \vec{S}_1 \hat{n} \cdot \vec{S}_2 (\hat{n} \cdot \vec{v}_2)^2 - 112 \hat{n} \cdot \vec{S}_1 \hat{n} \cdot \vec{S}_2 \hat{n} \cdot \vec{v}_1 \hat{n} \cdot \vec{v}_2 + 16 \hat{n} \cdot \vec{S}_2 \hat{n} \cdot \vec{v}_2 \vec{S}_1 \cdot \vec{v}_1 - 4 \hat{n} \cdot \vec{S}_2 \hat{n} \cdot \vec{v}_2 \vec{S}_1 \cdot \vec{v}_2 + \right. \right. \\ \left. \left. 16 \hat{n} \cdot \vec{S}_1 \hat{n} \cdot \vec{v}_2 \vec{S}_2 \cdot \vec{v}_1 - 4 \hat{n} \cdot \vec{S}_1 \hat{n} \cdot \vec{v}_2 \vec{S}_2 \cdot \vec{v}_2 + 20 \hat{n} \cdot \vec{S}_2 \hat{n} \cdot \vec{v}_1 \vec{S}_1 \cdot \vec{v}_2 + 20 \hat{n} \cdot \vec{S}_1 \hat{n} \cdot \vec{v}_1 \vec{S}_2 \cdot \vec{v}_2 + \right. \right. \\ \left. \left. 16 \vec{v}_1 \cdot \vec{v}_2 \hat{n} \cdot \vec{S}_1 \hat{n} \cdot \vec{S}_2 - 4 \vec{S}_1 \cdot \vec{v}_2 \vec{S}_2 \cdot \vec{v}_1 - 4 \vec{S}_1 \cdot \vec{v}_1 \vec{S}_2 \cdot \vec{v}_2 \right) + \frac{1}{r^4} \left( -20 \hat{n} \cdot \vec{S}_2 \hat{n} \cdot \vec{S}_1 \hat{n} \cdot \vec{v}_1 + 4 \hat{n} \cdot \vec{S}_2 \hat{n} \cdot \vec{S}_1 \hat{n} \cdot \vec{v}_2 + \right. \right. \\ \left. \left. 16 \hat{n} \cdot \vec{S}_2 \hat{n} \cdot \vec{S}_1 \hat{n} \cdot \vec{v}_2 - 4 \hat{n} \cdot \vec{S}_1 \hat{n} \cdot \vec{S}_2 \hat{n} \cdot \vec{v}_2 - 4 \hat{n} \cdot \vec{S}_1 \hat{n} \cdot \vec{S}_2 \hat{n} \cdot \vec{v}_2 \right) \right) \Bigg\}$$

$$16 \hat{n} \cdot \vec{S}_1 \hat{n} \cdot \vec{S}_2 \hat{n} \cdot \vec{v}_2 - 4 \hat{n} \cdot \vec{S}_2 \vec{S}_1 \cdot \vec{v}_2 + 4 \hat{n} \cdot \vec{S}_1 \vec{S}_2 \cdot \vec{v}_1 + 4 \hat{n} \cdot \vec{S}_2 \vec{S}_1 \cdot \vec{v}_1 - 4 \hat{n} \cdot \vec{S}_1 \vec{S}_2 \cdot \vec{v}_2 \Big) + \frac{4 \hat{n} \cdot \vec{S}_1 \hat{n} \cdot \vec{S}_2}{r^3} \Bigg\}$$

{DiagS1S2[3, 2, 36],

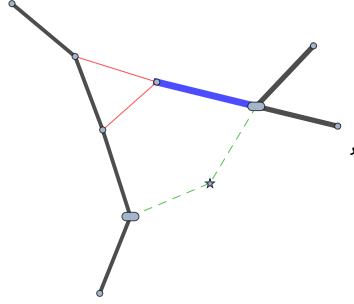

$$G^3 m_2^2 \left\{ \frac{1}{r^5} \left( \frac{1}{2} \hat{n} \times \vec{S}_1 \cdot \vec{v}_2 \hat{n} \times \vec{S}_2 \cdot \vec{v}_2 - \frac{15}{4} \hat{n} \cdot \vec{S}_1 \hat{n} \cdot \vec{S}_2 (\hat{n} \cdot \vec{v}_2)^2 + \frac{21}{2} \hat{n} \cdot \vec{S}_1 \hat{n} \cdot \vec{S}_2 \hat{n} \cdot \vec{v}_1 \hat{n} \cdot \vec{v}_2 + \frac{5}{4} \vec{S}_1 \cdot \vec{S}_2 \hat{n} \cdot \vec{v}_1 \hat{n} \cdot \vec{v}_2 - \right. \right. \\ \frac{3}{2} \hat{n} \cdot \vec{S}_2 \hat{n} \cdot \vec{v}_2 \vec{S}_1 \cdot \vec{v}_1 + \frac{3}{4} \hat{n} \cdot \vec{S}_2 \hat{n} \cdot \vec{v}_2 \vec{S}_1 \cdot \vec{v}_2 - \frac{3}{2} \hat{n} \cdot \vec{S}_1 \hat{n} \cdot \vec{v}_2 \vec{S}_2 \cdot \vec{v}_1 + \hat{n} \cdot \vec{S}_1 \hat{n} \cdot \vec{v}_2 \vec{S}_2 \cdot \vec{v}_2 - \\ \frac{5}{4} \hat{n} \cdot \vec{S}_2 \hat{n} \cdot \vec{v}_1 \vec{S}_1 \cdot \vec{v}_2 - \frac{5}{2} \hat{n} \cdot \vec{S}_1 \hat{n} \cdot \vec{v}_1 \vec{S}_2 \cdot \vec{v}_2 - \frac{3}{2} \vec{v}_1 \cdot \vec{v}_2 \hat{n} \cdot \vec{S}_1 \hat{n} \cdot \vec{S}_2 + \frac{1}{4} \vec{v}_2 \cdot \vec{v}_2 \hat{n} \cdot \vec{S}_1 \hat{n} \cdot \vec{S}_2 + \\ \left. \frac{1}{4} \vec{S}_1 \cdot \vec{v}_2 \vec{S}_2 \cdot \vec{v}_1 + \frac{1}{2} \vec{S}_1 \cdot \vec{v}_1 \vec{S}_2 \cdot \vec{v}_2 + \frac{1}{4} \vec{S}_1 \cdot \vec{v}_2 \vec{S}_2 \cdot \vec{v}_2 - \frac{1}{4} \vec{S}_1 \cdot \vec{S}_2 \vec{v}_1 \cdot \vec{v}_2 - \frac{1}{2} \vec{S}_1 \cdot \vec{S}_2 \vec{v}_2 \cdot \vec{v}_2 \right) + \\ \frac{1}{r^4} \left( \frac{15}{4} \hat{n} \cdot \vec{S}_2 \hat{n} \cdot \vec{S}_1 \hat{n} \cdot \vec{v}_1 + \frac{3}{4} \vec{S}_1 \cdot \vec{S}_2 \hat{n} \cdot \vec{v}_1 - \frac{9}{4} \hat{n} \cdot \vec{S}_2 \hat{n} \cdot \vec{S}_1 \hat{n} \cdot \vec{v}_2 - \frac{3}{2} \hat{n} \cdot \vec{S}_1 \hat{n} \cdot \vec{S}_2 \hat{n} \cdot \vec{v}_2 - \right. \\ \frac{1}{4} \vec{S}_1 \cdot \vec{S}_2 \hat{n} \cdot \vec{v}_2 + \frac{1}{4} \hat{n} \cdot \vec{S}_2 \vec{S}_1 \cdot \vec{v}_2 - \frac{3}{4} \hat{n} \cdot \vec{S}_1 \vec{S}_2 \cdot \vec{v}_1 + \frac{1}{4} \hat{n} \cdot \vec{S}_1 \vec{S}_2 \cdot \vec{v}_2 - \frac{1}{2} \vec{S}_1 \cdot \vec{S}_2 \hat{n} \cdot \vec{v}_2 - \\ \left. \frac{3}{4} \hat{n} \cdot \vec{S}_2 \vec{S}_1 \cdot \vec{v}_1 + \frac{1}{2} \hat{n} \cdot \vec{S}_2 \vec{S}_1 \cdot \vec{v}_2 + \frac{1}{2} \hat{n} \cdot \vec{S}_1 \vec{S}_2 \cdot \vec{v}_2 \right) + \frac{-\frac{3}{4} \hat{n} \cdot \vec{S}_1 \hat{n} \cdot \vec{S}_2 - \frac{1}{4} \vec{S}_1 \cdot \vec{S}_2}{r^3} \Bigg\}$$

{DiagS1S2[3, 2, 37],

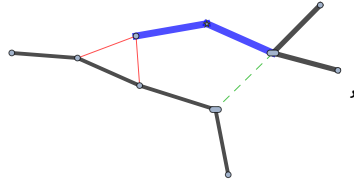

$$G^3 m_2^2 \left\{ \frac{1}{r^5} \left( \frac{1}{2} \hat{n} \times \vec{S}_1 \cdot \vec{v}_2 \hat{n} \times \vec{S}_2 \cdot \vec{v}_2 - \frac{41}{4} \hat{n} \cdot \vec{S}_1 \hat{n} \cdot \vec{S}_2 (\hat{n} \cdot \vec{v}_2)^2 + \frac{5}{2} \vec{S}_1 \cdot \vec{S}_2 (\hat{n} \cdot \vec{v}_2)^2 + \frac{175}{12} \hat{n} \cdot \vec{S}_1 \hat{n} \cdot \vec{S}_2 \hat{n} \cdot \vec{v}_1 \hat{n} \cdot \vec{v}_2 - \right. \right. \\ \frac{10}{3} \vec{S}_1 \cdot \vec{S}_2 \hat{n} \cdot \vec{v}_1 \hat{n} \cdot \vec{v}_2 - \frac{25}{12} \hat{n} \cdot \vec{S}_2 \hat{n} \cdot \vec{v}_2 \vec{S}_1 \cdot \vec{v}_1 + \frac{9}{4} \hat{n} \cdot \vec{S}_2 \hat{n} \cdot \vec{v}_2 \vec{S}_1 \cdot \vec{v}_2 - \frac{25}{12} \hat{n} \cdot \vec{S}_1 \hat{n} \cdot \vec{v}_2 \vec{S}_2 \cdot \vec{v}_1 + \\ \frac{3}{2} \hat{n} \cdot \vec{S}_1 \hat{n} \cdot \vec{v}_2 \vec{S}_2 \cdot \vec{v}_2 - \frac{5}{6} \hat{n} \cdot \vec{S}_2 \hat{n} \cdot \vec{v}_1 \vec{S}_1 \cdot \vec{v}_2 + \frac{5}{12} \hat{n} \cdot \vec{S}_1 \hat{n} \cdot \vec{v}_1 \vec{S}_2 \cdot \vec{v}_2 - \frac{25}{12} \vec{v}_1 \cdot \vec{v}_2 \hat{n} \cdot \vec{S}_1 \hat{n} \cdot \vec{S}_2 + \\ \frac{1}{4} \vec{v}_2 \cdot \vec{v}_2 \hat{n} \cdot \vec{S}_1 \hat{n} \cdot \vec{S}_2 + \frac{1}{6} \vec{S}_1 \cdot \vec{v}_2 \vec{S}_2 \cdot \vec{v}_1 - \frac{1}{12} \vec{S}_1 \cdot \vec{v}_1 \vec{S}_2 \cdot \vec{v}_2 + \frac{1}{4} \vec{S}_1 \cdot \vec{v}_2 \vec{S}_2 \cdot \vec{v}_2 + \frac{2}{3} \vec{S}_1 \cdot \vec{S}_2 \vec{v}_1 \cdot \vec{v}_2 - \frac{1}{2} \vec{S}_1 \cdot \vec{S}_2 \vec{v}_2 \cdot \vec{v}_2 \Big) + \\ \frac{1}{r^4} \left( -\frac{25}{12} \hat{n} \cdot \vec{S}_2 \hat{n} \cdot \vec{S}_1 \hat{n} \cdot \vec{v}_2 - \frac{25}{12} \hat{n} \cdot \vec{S}_1 \hat{n} \cdot \vec{S}_2 \hat{n} \cdot \vec{v}_2 + \frac{2}{3} \vec{S}_1 \cdot \vec{S}_2 \hat{n} \cdot \vec{v}_2 + \frac{2}{3} \vec{S}_1 \cdot \vec{S}_2 \hat{n} \cdot \vec{v}_2 + \right. \\ \left. \frac{1}{6} \hat{n} \cdot \vec{S}_2 \vec{S}_1 \cdot \vec{v}_2 - \frac{1}{12} \hat{n} \cdot \vec{S}_1 \vec{S}_2 \cdot \vec{v}_2 + \frac{1}{6} \hat{n} \cdot \vec{S}_2 \vec{S}_1 \cdot \vec{v}_2 - \frac{1}{12} \hat{n} \cdot \vec{S}_1 \vec{S}_2 \cdot \vec{v}_2 \right) \Bigg\}$$

{DiagS1S2 [3, 2, 38],

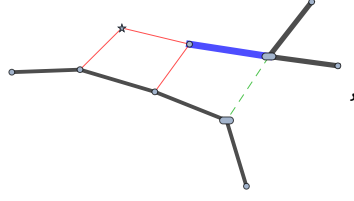

$$G^3 m_2^2 \left( \frac{1}{r^5} \left( \hat{n} \times \vec{S}_1 \cdot \vec{v}_2 \hat{n} \times \vec{S}_2 \cdot \vec{v}_2 + \frac{1}{3} \hat{n} \cdot \vec{S}_1 \hat{n} \cdot \vec{S}_2 (\hat{n} \cdot \vec{v}_2)^2 + \frac{13}{6} \vec{S}_1 \cdot \vec{S}_2 (\hat{n} \cdot \vec{v}_2)^2 - \frac{7}{6} \hat{n} \cdot \vec{S}_1 \hat{n} \cdot \vec{S}_2 \hat{n} \cdot \vec{v}_1 \hat{n} \cdot \vec{v}_2 - \right. \right. \\ \left. \frac{5}{6} \vec{S}_1 \cdot \vec{S}_2 \hat{n} \cdot \vec{v}_1 \hat{n} \cdot \vec{v}_2 + \frac{1}{6} \hat{n} \cdot \vec{S}_2 \hat{n} \cdot \vec{v}_2 \vec{S}_1 \cdot \vec{v}_1 + \frac{17}{6} \hat{n} \cdot \vec{S}_2 \hat{n} \cdot \vec{v}_2 \vec{S}_1 \cdot \vec{v}_2 + \frac{1}{6} \hat{n} \cdot \vec{S}_1 \hat{n} \cdot \vec{v}_2 \vec{S}_2 \cdot \vec{v}_1 - \right. \\ \left. \frac{8}{3} \hat{n} \cdot \vec{S}_1 \hat{n} \cdot \vec{v}_2 \vec{S}_2 \cdot \vec{v}_2 - \frac{10}{3} \hat{n} \cdot \vec{S}_2 \hat{n} \cdot \vec{v}_1 \vec{S}_1 \cdot \vec{v}_2 + \frac{5}{3} \hat{n} \cdot \vec{S}_1 \hat{n} \cdot \vec{v}_1 \vec{S}_2 \cdot \vec{v}_2 + \frac{1}{6} \vec{v}_1 \cdot \vec{v}_2 \hat{n} \cdot \vec{S}_1 \hat{n} \cdot \vec{S}_2 - \right. \\ \left. \frac{5}{6} \vec{v}_2 \cdot \vec{v}_2 \hat{n} \cdot \vec{S}_1 \hat{n} \cdot \vec{S}_2 + \frac{2}{3} \vec{S}_1 \cdot \vec{v}_2 \vec{S}_2 \cdot \vec{v}_1 - \frac{1}{3} \vec{S}_1 \cdot \vec{v}_1 \vec{S}_2 \cdot \vec{v}_2 + \frac{1}{3} \vec{S}_1 \cdot \vec{v}_2 \vec{S}_2 \cdot \vec{v}_2 + \frac{1}{6} \vec{S}_1 \cdot \vec{S}_2 \vec{v}_1 \cdot \vec{v}_2 - \frac{5}{6} \vec{S}_1 \cdot \vec{S}_2 \vec{v}_2 \cdot \vec{v}_2 \right) + \\ \left. \frac{1}{r^4} \left( \frac{1}{6} \hat{n} \cdot \vec{S}_2 \hat{n} \cdot \vec{S}_1 \hat{n} \cdot \vec{v}_2 + \frac{1}{6} \hat{n} \cdot \vec{S}_1 \hat{n} \cdot \vec{S}_2 \hat{n} \cdot \vec{v}_2 + \frac{1}{6} \vec{S}_1 \cdot \vec{S}_2 \hat{n} \cdot \vec{v}_2 + \frac{1}{6} \vec{S}_1 \cdot \vec{S}_2 \hat{n} \cdot \vec{v}_2 + \right. \right. \\ \left. \left. \frac{2}{3} \hat{n} \cdot \vec{S}_2 \vec{S}_1 \cdot \vec{v}_2 - \frac{1}{3} \hat{n} \cdot \vec{S}_1 \vec{S}_2 \cdot \vec{v}_2 + \frac{2}{3} \hat{n} \cdot \vec{S}_2 \vec{S}_1 \cdot \vec{v}_2 - \frac{1}{3} \hat{n} \cdot \vec{S}_1 \vec{S}_2 \cdot \vec{v}_2 \right) \right) \Bigg\}$$

{DiagS1S2 [3, 2, 39],

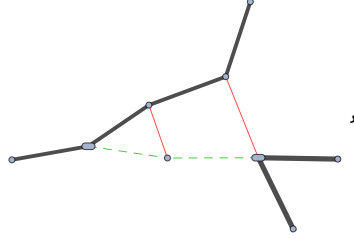

$$G^3 m_2^2 \left( \frac{-32 \vec{S}_1 \cdot \vec{a}_2 \hat{n} \cdot \vec{S}_2 + 32 \vec{S}_1 \cdot \vec{S}_2 \hat{n} \cdot \vec{a}_2 + 32 \vec{S}_1 \cdot \vec{S}_2 \hat{n} \cdot \vec{v}_2 - 32 \hat{n} \cdot \vec{S}_2 \vec{S}_1 \cdot \vec{v}_2}{r^4} + \frac{1}{r^5} \right. \\ \left. (-56 \hat{n} \times \vec{S}_1 \cdot \vec{v}_2 \hat{n} \times \vec{S}_2 \cdot \vec{v}_2 + 40 \vec{S}_1 \cdot \vec{S}_2 (\hat{n} \cdot \vec{v}_2)^2 + 4 \vec{S}_1 \cdot \vec{S}_2 \hat{n} \cdot \vec{v}_1 \hat{n} \cdot \vec{v}_2 - 40 \hat{n} \cdot \vec{S}_2 \hat{n} \cdot \vec{v}_2 \vec{S}_1 \cdot \vec{v}_2 - \right. \\ \left. 4 \hat{n} \cdot \vec{S}_1 \hat{n} \cdot \vec{v}_2 \vec{S}_2 \cdot \vec{v}_1 + 48 \vec{v}_2 \cdot \vec{v}_2 \hat{n} \cdot \vec{S}_1 \hat{n} \cdot \vec{S}_2 - 4 \vec{S}_1 \cdot \vec{v}_2 \vec{S}_2 \cdot \vec{v}_2 - 20 \vec{S}_1 \cdot \vec{S}_2 \vec{v}_2 \cdot \vec{v}_2) \right) \Bigg\}$$

{DiagS1S2 [3, 2, 40],

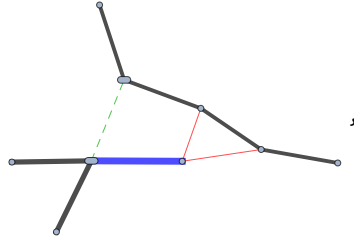

$$G^3 m_2^2 \left( \frac{\vec{S}_1 \cdot \vec{a}_2 \hat{n} \cdot \vec{S}_2 - \vec{S}_1 \cdot \vec{S}_2 \hat{n} \cdot \vec{a}_2 + \hat{n} \cdot \vec{S}_2 \hat{n} \cdot \vec{S}_1 \hat{n} \cdot \vec{v}_1 - \vec{S}_1 \cdot \vec{S}_2 \hat{n} \cdot \vec{v}_1 - \vec{S}_1 \cdot \vec{S}_2 \hat{n} \cdot \vec{v}_2 + \hat{n} \cdot \vec{S}_2 \vec{S}_1 \cdot \vec{v}_2}{r^4} + \frac{1}{r^5} \right. \\ \left( -\frac{3}{4} \hat{n} \times \vec{S}_1 \cdot \vec{v}_1 \hat{n} \times \vec{S}_2 \cdot \vec{v}_1 - \hat{n} \times \vec{S}_1 \cdot \vec{v}_1 \hat{n} \times \vec{S}_2 \cdot \vec{v}_2 + \frac{11}{4} \hat{n} \times \vec{S}_1 \cdot \vec{v}_2 \hat{n} \times \vec{S}_2 \cdot \vec{v}_2 - \frac{9}{4} \hat{n} \cdot \vec{S}_1 \hat{n} \cdot \vec{S}_2 (\hat{n} \cdot \vec{v}_1)^2 + \right. \\ \left. \frac{3}{4} \vec{S}_1 \cdot \vec{S}_2 (\hat{n} \cdot \vec{v}_1)^2 - \hat{n} \cdot \vec{S}_1 \hat{n} \cdot \vec{S}_2 \hat{n} \cdot \vec{v}_2 \hat{n} \cdot \vec{v}_1 - \vec{S}_1 \cdot \vec{S}_2 \hat{n} \cdot \vec{v}_2 \hat{n} \cdot \vec{v}_1 + \frac{3}{2} \hat{n} \cdot \vec{S}_2 \hat{n} \cdot \vec{v}_1 \vec{S}_1 \cdot \vec{v}_1 - \hat{n} \cdot \vec{S}_2 \hat{n} \cdot \vec{v}_1 \vec{S}_1 \cdot \vec{v}_2 + \right. \\ \left. \hat{n} \cdot \vec{S}_1 \hat{n} \cdot \vec{v}_1 \vec{S}_2 \cdot \vec{v}_2 - 3 \hat{n} \cdot \vec{S}_1 \hat{n} \cdot \vec{S}_2 (\hat{n} \cdot \vec{v}_2)^2 + \frac{3}{4} \vec{S}_1 \cdot \vec{S}_2 (\hat{n} \cdot \vec{v}_2)^2 + \frac{1}{4} \hat{n} \cdot \vec{S}_2 \hat{n} \cdot \vec{v}_2 \vec{S}_1 \cdot \vec{v}_2 + 2 \hat{n} \cdot \vec{S}_1 \hat{n} \cdot \vec{v}_2 \vec{S}_2 \cdot \vec{v}_1 + \right. \\ \left. \frac{1}{4} \hat{n} \cdot \vec{S}_2 \hat{n} \cdot \vec{v}_2 \vec{S}_2 \cdot \vec{v}_1 \right) \Bigg\}$$

$$\left. \left. \left. \vec{v}_1 \cdot \vec{v}_2 \hat{n} \cdot \vec{S}_1 \hat{n} \cdot \vec{S}_2 - \frac{9}{2} \vec{v}_2 \cdot \vec{v}_2 \hat{n} \cdot \vec{S}_1 \hat{n} \cdot \vec{S}_2 + \vec{S}_1 \cdot \vec{v}_2 \vec{S}_2 \cdot \vec{v}_2 - \vec{S}_1 \cdot \vec{S}_2 \vec{v}_1 \cdot \vec{v}_2 - \frac{1}{2} \vec{S}_1 \cdot \vec{S}_2 \vec{v}_2 \cdot \vec{v}_2 \right) \right\} \right\}$$

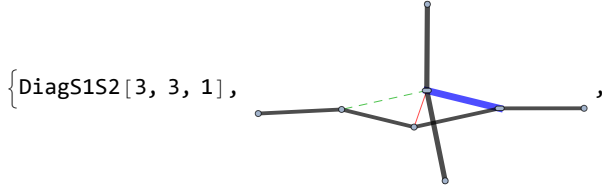

$$\frac{G^3 m_2^2 \left( -24 \hat{n} \times \vec{S}_1 \cdot \vec{v}_2 \hat{n} \times \vec{S}_2 \cdot \vec{v}_2 - 8 \vec{S}_1 \cdot \vec{S}_2 (\hat{n} \cdot \vec{v}_2)^2 + 8 \hat{n} \cdot \vec{S}_1 \hat{n} \cdot \vec{v}_2 \vec{S}_2 \cdot \vec{v}_2 - 8 \vec{v}_2 \cdot \vec{v}_2 \hat{n} \cdot \vec{S}_1 \hat{n} \cdot \vec{S}_2 + 8 \vec{S}_1 \cdot \vec{S}_2 \vec{v}_2 \cdot \vec{v}_2 \right)}{r^5} \Bigg\}$$

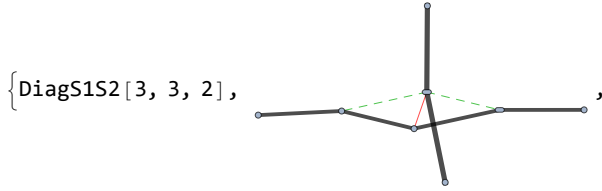

$$G^3 m_2^2 \left( \frac{16 \vec{S}_1 \cdot \vec{S}_2 \hat{n} \cdot \vec{a}_2 - 16 \vec{S}_2 \cdot \vec{a}_2 \hat{n} \cdot \vec{S}_1 + 16 \hat{n} \cdot \vec{S}_1 \vec{S}_2 \cdot \vec{v}_2 - 16 \vec{S}_1 \cdot \vec{S}_2 \hat{n} \cdot \vec{v}_2}{r^4} + \right. \\ \left. \frac{1}{r^5} \left( -16 \hat{n} \times \vec{S}_1 \cdot \vec{v}_2 \hat{n} \times \vec{S}_2 \cdot \vec{v}_1 - 32 \vec{S}_1 \cdot \vec{S}_2 (\hat{n} \cdot \vec{v}_2)^2 + 32 \hat{n} \cdot \vec{S}_1 \hat{n} \cdot \vec{v}_2 \vec{S}_2 \cdot \vec{v}_2 + \right. \right. \\ \left. \left. 48 \vec{v}_1 \cdot \vec{v}_2 \hat{n} \cdot \vec{S}_1 \hat{n} \cdot \vec{S}_2 - 16 \vec{S}_1 \cdot \vec{v}_2 \vec{S}_2 \cdot \vec{v}_2 - 16 \vec{S}_1 \cdot \vec{S}_2 \vec{v}_1 \cdot \vec{v}_2 + 16 \vec{S}_1 \cdot \vec{S}_2 \vec{v}_2 \cdot \vec{v}_2 \right) \right) \Bigg\}$$

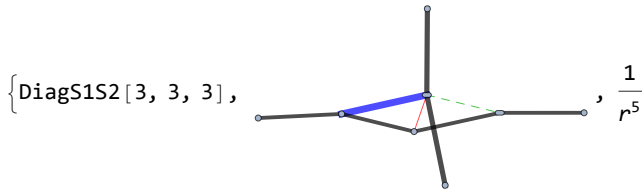

$$G^3 m_2^2 \left( 24 \hat{n} \times \vec{S}_1 \cdot \vec{v}_2 \hat{n} \times \vec{S}_2 \cdot \vec{v}_2 + 24 \vec{S}_1 \cdot \vec{S}_2 (\hat{n} \cdot \vec{v}_2)^2 - 24 \hat{n} \cdot \vec{S}_1 \hat{n} \cdot \vec{v}_2 \vec{S}_2 \cdot \vec{v}_2 + \right. \\ \left. 48 \vec{v}_2 \cdot \vec{v}_2 \hat{n} \cdot \vec{S}_1 \hat{n} \cdot \vec{S}_2 + 16 \vec{S}_1 \cdot \vec{v}_2 \vec{S}_2 \cdot \vec{v}_2 - 32 \vec{S}_1 \cdot \vec{S}_2 \vec{v}_2 \cdot \vec{v}_2 \right) \Bigg\}$$

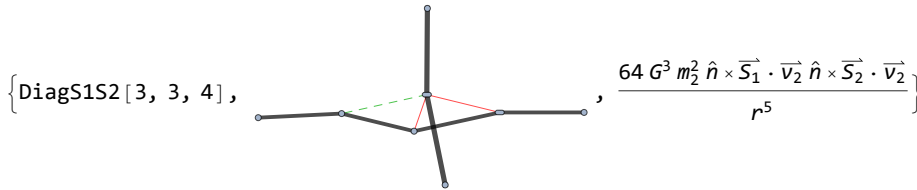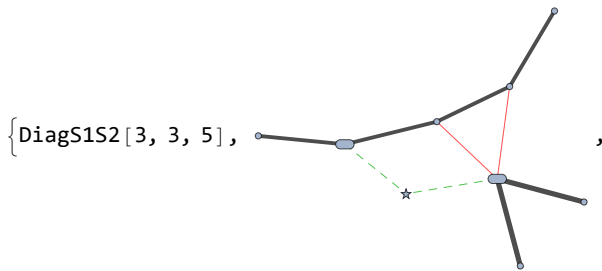

$$G^3 m_2^2 \left\{ \frac{1}{r^5} \left( -24 \hat{n} \cdot \vec{S}_1 \hat{n} \cdot \vec{S}_2 (\hat{n} \cdot \vec{v}_2)^2 - 8 \vec{S}_1 \cdot \vec{S}_2 (\hat{n} \cdot \vec{v}_2)^2 + 84 \hat{n} \cdot \vec{S}_1 \hat{n} \cdot \vec{S}_2 \hat{n} \cdot \vec{v}_1 \hat{n} \cdot \vec{v}_2 + 20 \vec{S}_1 \cdot \vec{S}_2 \hat{n} \cdot \vec{v}_1 \hat{n} \cdot \vec{v}_2 - \right. \right. \\ \left. \left. 12 \hat{n} \cdot \vec{S}_2 \hat{n} \cdot \vec{v}_2 \vec{S}_1 \cdot \vec{v}_1 + 8 \hat{n} \cdot \vec{S}_2 \hat{n} \cdot \vec{v}_2 \vec{S}_1 \cdot \vec{v}_2 - 12 \hat{n} \cdot \vec{S}_1 \hat{n} \cdot \vec{v}_2 \vec{S}_2 \cdot \vec{v}_1 + 8 \hat{n} \cdot \vec{S}_1 \hat{n} \cdot \vec{v}_2 \vec{S}_2 \cdot \vec{v}_2 - 20 \hat{n} \cdot \vec{S}_2 \hat{n} \cdot \vec{v}_1 \vec{S}_1 \cdot \vec{v}_2 - \right. \right. \\ \left. \left. 20 \hat{n} \cdot \vec{S}_1 \hat{n} \cdot \vec{v}_1 \vec{S}_2 \cdot \vec{v}_2 - 12 \vec{v}_1 \cdot \vec{v}_2 \hat{n} \cdot \vec{S}_1 \hat{n} \cdot \vec{S}_2 + 4 \vec{S}_1 \cdot \vec{v}_2 \vec{S}_2 \cdot \vec{v}_1 + 4 \vec{S}_1 \cdot \vec{v}_1 \vec{S}_2 \cdot \vec{v}_2 - 4 \vec{S}_1 \cdot \vec{S}_2 \vec{v}_1 \cdot \vec{v}_2 \right) + \frac{1}{r^4} \right. \\ \left. \left( 20 \hat{n} \cdot \vec{S}_2 \hat{n} \cdot \vec{S}_1 \hat{n} \cdot \vec{v}_1 + 12 \vec{S}_1 \cdot \vec{S}_2 \hat{n} \cdot \vec{v}_1 - 8 \hat{n} \cdot \vec{S}_2 \hat{n} \cdot \vec{S}_1 \hat{n} \cdot \vec{v}_2 - 12 \hat{n} \cdot \vec{S}_1 \hat{n} \cdot \vec{S}_2 \hat{n} \cdot \vec{v}_2 - 4 \vec{S}_1 \cdot \vec{S}_2 \hat{n} \cdot \vec{v}_2 + \right. \right. \\ \left. \left. 4 \hat{n} \cdot \vec{S}_2 \vec{S}_1 \cdot \vec{v}_2 - 4 \hat{n} \cdot \vec{S}_1 \vec{S}_2 \cdot \vec{v}_1 - 8 \vec{S}_1 \cdot \vec{S}_2 \hat{n} \cdot \vec{v}_2 - 4 \hat{n} \cdot \vec{S}_2 \vec{S}_1 \cdot \vec{v}_1 + 4 \hat{n} \cdot \vec{S}_1 \vec{S}_2 \cdot \vec{v}_2 \right) + \frac{-4 \hat{n} \cdot \vec{S}_1 \hat{n} \cdot \vec{S}_2 - 4 \vec{S}_1 \cdot \vec{S}_2}{r^3} \right\}$$

{DiagS1S2 [3, 3, 6],

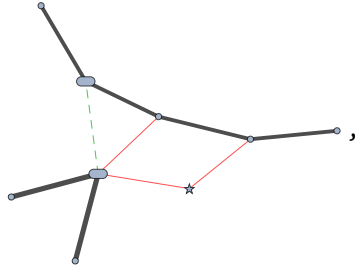

$$G^3 m_2^2 \left\{ \frac{1}{r^5} \left( -144 \hat{n} \cdot \vec{S}_1 \hat{n} \cdot \vec{S}_2 (\hat{n} \cdot \vec{v}_2)^2 + 32 \vec{S}_1 \cdot \vec{S}_2 (\hat{n} \cdot \vec{v}_2)^2 + 168 \hat{n} \cdot \vec{S}_1 \hat{n} \cdot \vec{S}_2 \hat{n} \cdot \vec{v}_1 \hat{n} \cdot \vec{v}_2 - \right. \right. \\ \left. \left. 40 \vec{S}_1 \cdot \vec{S}_2 \hat{n} \cdot \vec{v}_1 \hat{n} \cdot \vec{v}_2 - 24 \hat{n} \cdot \vec{S}_2 \hat{n} \cdot \vec{v}_2 \vec{S}_1 \cdot \vec{v}_1 + 24 \hat{n} \cdot \vec{S}_2 \hat{n} \cdot \vec{v}_2 \vec{S}_1 \cdot \vec{v}_2 - \right. \right. \\ \left. \left. 24 \hat{n} \cdot \vec{S}_1 \hat{n} \cdot \vec{v}_2 \vec{S}_2 \cdot \vec{v}_1 + 24 \hat{n} \cdot \vec{S}_1 \hat{n} \cdot \vec{v}_2 \vec{S}_2 \cdot \vec{v}_2 - 24 \vec{v}_1 \cdot \vec{v}_2 \hat{n} \cdot \vec{S}_1 \hat{n} \cdot \vec{S}_2 + 8 \vec{S}_1 \cdot \vec{S}_2 \vec{v}_1 \cdot \vec{v}_2 \right) + \right. \\ \left. \frac{-24 \hat{n} \cdot \vec{S}_2 \hat{n} \cdot \vec{S}_1 \hat{n} \cdot \vec{v}_2 - 24 \hat{n} \cdot \vec{S}_1 \hat{n} \cdot \vec{S}_2 \hat{n} \cdot \vec{v}_2 + 8 \vec{S}_1 \cdot \vec{S}_2 \hat{n} \cdot \vec{v}_2 + 8 \vec{S}_1 \cdot \vec{S}_2 \hat{n} \cdot \vec{v}_2}{r^4} \right\}$$

{DiagS1S2 [3, 3, 7],

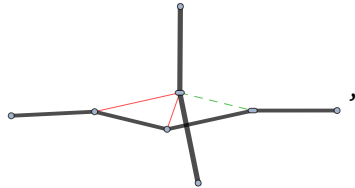

$$G^3 m_2^2 \left\{ \frac{16 \vec{S}_1 \cdot \vec{a}_2 \hat{n} \cdot \vec{S}_2 - 16 \vec{S}_1 \cdot \vec{S}_2 \hat{n} \cdot \vec{a}_2 - 16 \vec{S}_1 \cdot \vec{S}_2 \hat{n} \cdot \vec{v}_2 + 16 \hat{n} \cdot \vec{S}_2 \vec{S}_1 \cdot \vec{v}_2}{r^4} + \frac{1}{r^5} \left( 36 \hat{n} \times \vec{S}_1 \cdot \vec{v}_2 \hat{n} \times \vec{S}_2 \cdot \vec{v}_2 - \right. \right. \\ \left. \left. 12 \vec{S}_1 \cdot \vec{S}_2 (\hat{n} \cdot \vec{v}_2)^2 + 12 \hat{n} \cdot \vec{S}_2 \hat{n} \cdot \vec{v}_2 \vec{S}_1 \cdot \vec{v}_2 - 72 \vec{v}_2 \cdot \vec{v}_2 \hat{n} \cdot \vec{S}_1 \hat{n} \cdot \vec{S}_2 + 8 \vec{S}_1 \cdot \vec{v}_2 \vec{S}_2 \cdot \vec{v}_2 + 16 \vec{S}_1 \cdot \vec{S}_2 \vec{v}_2 \cdot \vec{v}_2 \right) \right\}$$

{DiagS1S2 [3, 4, 1],

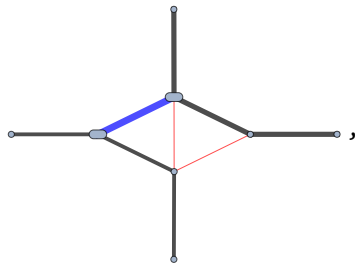



$$\frac{G^3 m_1 m_2 \left( 2 \hat{n} \times \vec{S}_1 \cdot \vec{v}_2 \hat{n} \times \vec{S}_2 \cdot \vec{v}_1 + 2 \vec{S}_1 \cdot \vec{S}_2 \hat{n} \cdot \vec{v}_1 \hat{n} \cdot \vec{v}_2 - 2 \hat{n} \cdot \vec{S}_1 \hat{n} \cdot \vec{v}_2 \vec{S}_2 \cdot \vec{v}_1 - 2 \vec{v}_1 \cdot \vec{v}_2 \hat{n} \cdot \vec{S}_1 \hat{n} \cdot \vec{S}_2 + 2 \vec{S}_1 \cdot \vec{S}_2 \vec{v}_1 \cdot \vec{v}_2 \right)}{r^5} \Bigg\}$$

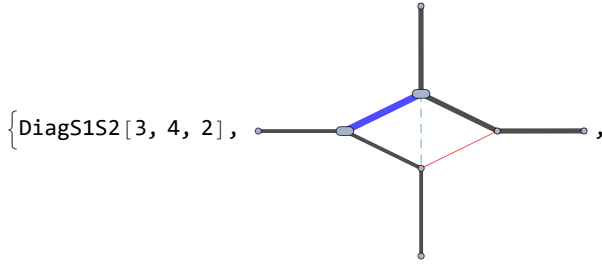

$$\frac{G^3 m_1 m_2 \left( -6 \hat{n} \times \vec{S}_1 \cdot \vec{v}_2 \hat{n} \times \vec{S}_2 \cdot \vec{v}_2 - 2 \vec{S}_1 \cdot \vec{S}_2 (\hat{n} \cdot \vec{v}_2)^2 + 2 \hat{n} \cdot \vec{S}_1 \hat{n} \cdot \vec{v}_2 \vec{S}_2 \cdot \vec{v}_2 - 2 \vec{v}_2 \cdot \vec{v}_2 \hat{n} \cdot \vec{S}_1 \hat{n} \cdot \vec{S}_2 + 2 \vec{S}_1 \cdot \vec{S}_2 \vec{v}_2 \cdot \vec{v}_2 \right)}{r^5} \Bigg\}$$

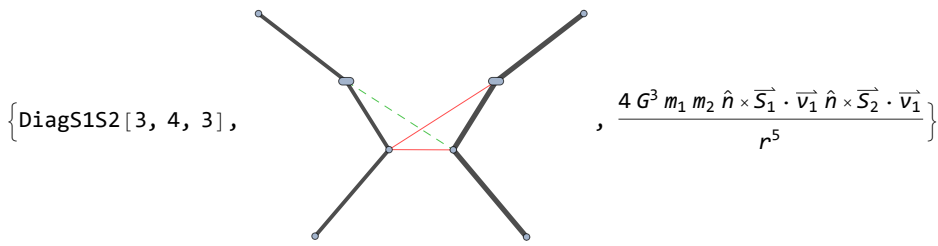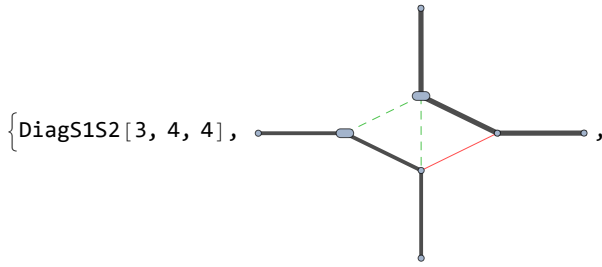

$$G^3 m_1 m_2 \left( \frac{4 \vec{S}_1 \cdot \vec{S}_2 \hat{n} \cdot \vec{a}_2 - 4 \vec{S}_2 \cdot \vec{a}_2 \hat{n} \cdot \vec{S}_1 + 4 \hat{n} \cdot \vec{S}_1 \vec{S}_2 \cdot \vec{v}_2 - 4 \vec{S}_1 \cdot \vec{S}_2 \hat{n} \cdot \vec{v}_2}{r^4} + \frac{1}{r^5} \right. \\ \left. \left( -4 \hat{n} \times \vec{S}_1 \cdot \vec{v}_2 \hat{n} \times \vec{S}_2 \cdot \vec{v}_1 - 4 \vec{S}_1 \cdot \vec{S}_2 (\hat{n} \cdot \vec{v}_2)^2 - 4 \vec{S}_1 \cdot \vec{S}_2 \hat{n} \cdot \vec{v}_1 \hat{n} \cdot \vec{v}_2 + 4 \hat{n} \cdot \vec{S}_1 \hat{n} \cdot \vec{v}_2 \vec{S}_2 \cdot \vec{v}_2 + \right. \right. \\ \left. \left. 4 \hat{n} \cdot \vec{S}_1 \hat{n} \cdot \vec{v}_1 \vec{S}_2 \cdot \vec{v}_2 + 12 \vec{v}_1 \cdot \vec{v}_2 \hat{n} \cdot \vec{S}_1 \hat{n} \cdot \vec{S}_2 - 4 \vec{S}_1 \cdot \vec{v}_2 \vec{S}_2 \cdot \vec{v}_2 - 4 \vec{S}_1 \cdot \vec{S}_2 \vec{v}_1 \cdot \vec{v}_2 + 4 \vec{S}_1 \cdot \vec{S}_2 \vec{v}_2 \cdot \vec{v}_2 \right) \right) \Bigg\}$$

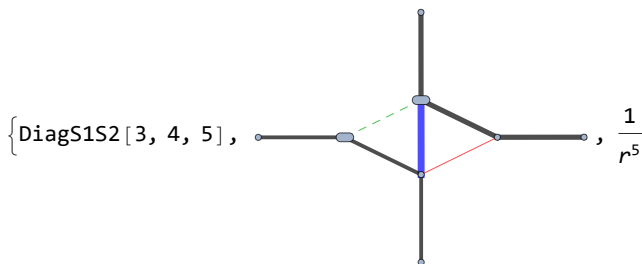

$$G^3 m_1 m_2 \left( -18 \hat{n} \times \vec{S}_1 \cdot \vec{v}_2 \hat{n} \times \vec{S}_2 \cdot \vec{v}_2 - 18 \vec{S}_1 \cdot \vec{S}_2 (\hat{n} \cdot \vec{v}_2)^2 + 18 \hat{n} \cdot \vec{S}_1 \hat{n} \cdot \vec{v}_2 \vec{S}_2 \cdot \vec{v}_2 - \right. \\ \left. 36 \vec{v}_2 \cdot \vec{v}_2 \hat{n} \cdot \vec{S}_1 \hat{n} \cdot \vec{S}_2 - 12 \vec{S}_1 \cdot \vec{v}_2 \vec{S}_2 \cdot \vec{v}_2 + 24 \vec{S}_1 \cdot \vec{S}_2 \vec{v}_2 \cdot \vec{v}_2 \right) \Bigg\}$$

$$\left\{ \text{DiagS1S2}[3, 4, 6], \right. , \left. \frac{G^3 m_1 m_2 \left( 48 \vec{v}_1 \cdot \vec{v}_2 \hat{n} \cdot \vec{S}_1 \hat{n} \cdot \vec{S}_2 - 16 \vec{S}_1 \cdot \vec{S}_2 \vec{v}_1 \cdot \vec{v}_2 \right)}{r^5} \right\}$$
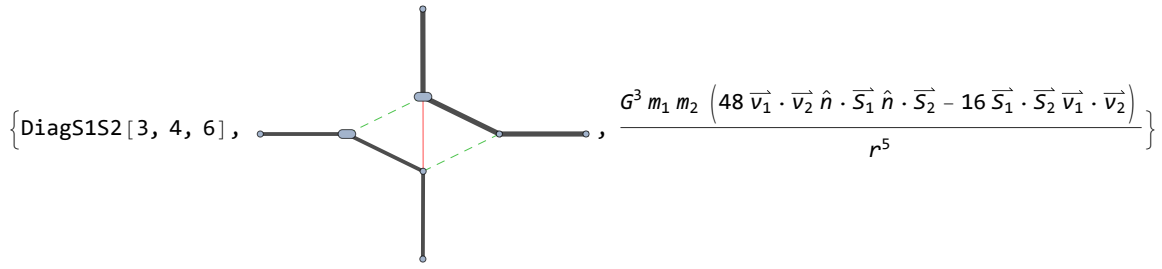

$$\left\{ \text{DiagS1S2}[3, 4, 7], \right. , \left. \frac{16 G^3 m_1 m_2 \hat{n} \times \vec{S}_1 \cdot \vec{v}_2 \hat{n} \times \vec{S}_2 \cdot \vec{v}_1}{r^5} \right\}$$
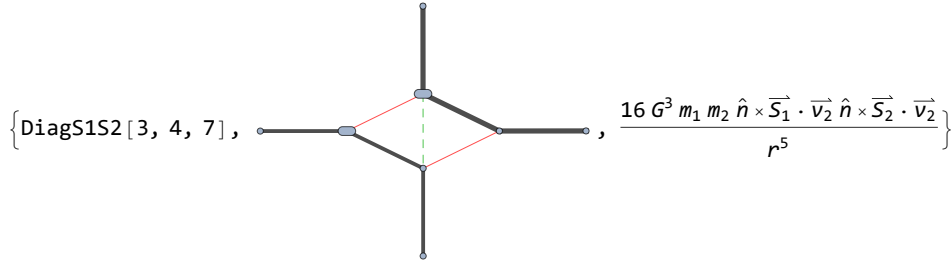

$$\left\{ \text{DiagS1S2}[3, 4, 8], \right. , \left. \frac{G^3 m_1 m_2 \left( -4 \hat{n} \cdot \vec{S}_2 \hat{n} \cdot \vec{v}_1 \vec{S}_1 \cdot \vec{v}_1 + 4 \hat{n} \cdot \vec{S}_1 \hat{n} \cdot \vec{v}_1 \vec{S}_2 \cdot \vec{v}_1 + 4 \vec{v}_1 \cdot \vec{v}_1 \hat{n} \cdot \vec{S}_1 \hat{n} \cdot \vec{S}_2 - 4 \vec{S}_2 \cdot \vec{v}_1 \vec{S}_1 \cdot \vec{v}_1 \right)}{r^5} \right\}$$
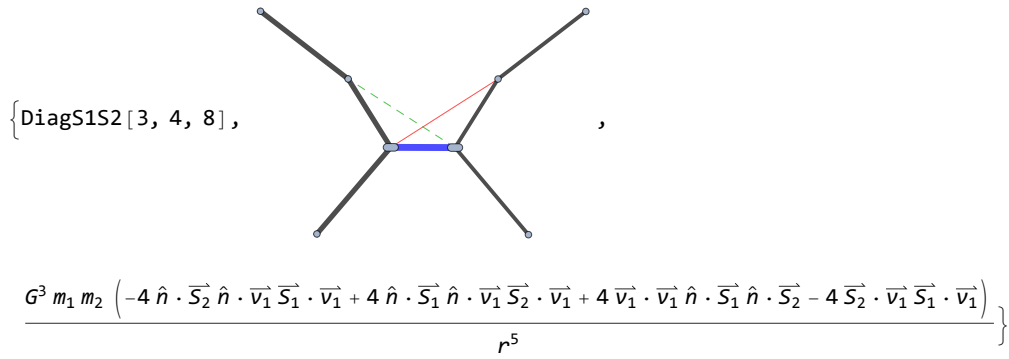

$$\left\{ \text{DiagS1S2}[3, 4, 9], \right. , \left. \frac{1}{r^5} \right\}$$
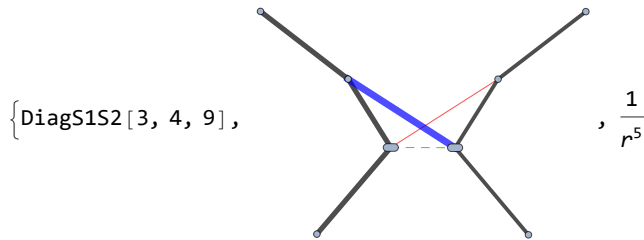

$$G^3 m_1 m_2 \left( 24 \hat{n} \times \vec{S}_1 \cdot \vec{v}_1 \hat{n} \times \vec{S}_2 \cdot \vec{v}_1 + 24 \vec{S}_1 \cdot \vec{S}_2 (\hat{n} \cdot \vec{v}_1)^2 - 24 \hat{n} \cdot \vec{S}_2 \hat{n} \cdot \vec{v}_1 \vec{S}_1 \cdot \vec{v}_1 + 48 \vec{v}_1 \cdot \vec{v}_1 \hat{n} \cdot \vec{S}_1 \hat{n} \cdot \vec{S}_2 + 16 \vec{S}_1 \cdot \vec{v}_1 \vec{S}_2 \cdot \vec{v}_1 - 32 \vec{S}_1 \cdot \vec{S}_2 \vec{v}_1 \cdot \vec{v}_1 \right) \}$$

$$\left\{ \text{DiagS1S2}[3, 4, 10], \right. , \left. \frac{16 \vec{S}_1 \cdot \vec{a}_1 \hat{n} \cdot \vec{S}_2 - 16 \vec{S}_1 \cdot \vec{S}_2 \hat{n} \cdot \vec{a}_1 + 16 \vec{S}_1 \cdot \vec{S}_2 \hat{n} \cdot \vec{v}_1 - 16 \hat{n} \cdot \vec{S}_2 \vec{S}_1 \cdot \vec{v}_1}{r^4} + \frac{1}{r^5} \right. \\ \left. \left( -16 \hat{n} \times \vec{S}_1 \cdot \vec{v}_2 \hat{n} \times \vec{S}_2 \cdot \vec{v}_1 - 48 \vec{S}_1 \cdot \vec{S}_2 (\hat{n} \cdot \vec{v}_1)^2 + 16 \vec{S}_1 \cdot \vec{S}_2 \hat{n} \cdot \vec{v}_2 \hat{n} \cdot \vec{v}_1 + 48 \hat{n} \cdot \vec{S}_2 \hat{n} \cdot \vec{v}_1 \vec{S}_1 \cdot \vec{v}_1 - \right. \right.$$
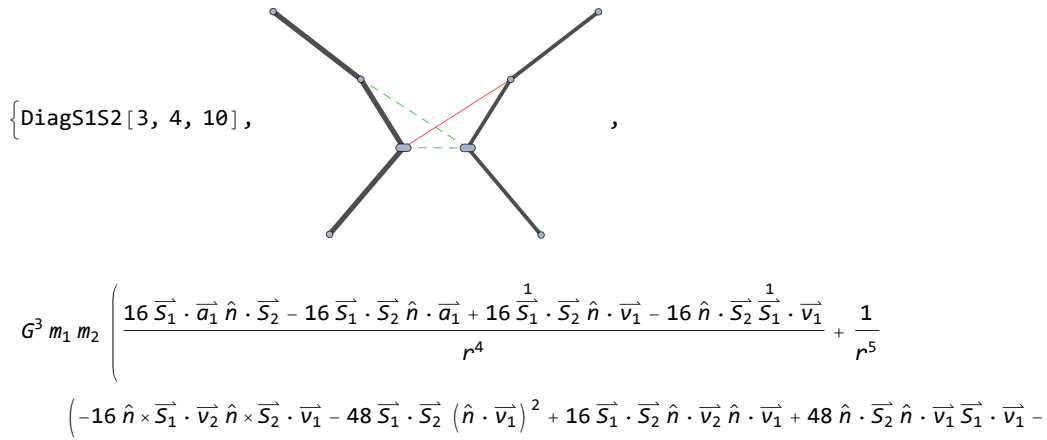

$$16 \hat{n} \cdot \vec{S}_2 \hat{n} \cdot \vec{v}_2 \vec{S}_1 \cdot \vec{v}_1 + 48 \vec{v}_1 \cdot \vec{v}_2 \hat{n} \cdot \vec{S}_1 \hat{n} \cdot \vec{S}_2 - 16 \vec{S}_1 \cdot \vec{v}_1 \vec{S}_2 \cdot \vec{v}_1 + 16 \vec{S}_1 \cdot \vec{S}_2 \vec{v}_1 \cdot \vec{v}_1 - 16 \vec{S}_1 \cdot \vec{S}_2 \vec{v}_1 \cdot \vec{v}_2 \Bigg) \Bigg\}$$

{DiagS1S2[3, 4, 11],

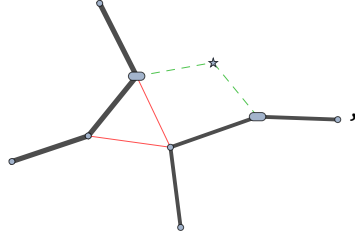

$$G^3 m_1 m_2 \left\{ \frac{1}{r^5} \left( -12 \hat{n} \cdot \vec{S}_1 \hat{n} \cdot \vec{S}_2 (\hat{n} \cdot \vec{v}_2)^2 - 4 \vec{S}_1 \cdot \vec{S}_2 (\hat{n} \cdot \vec{v}_2)^2 + 42 \hat{n} \cdot \vec{S}_1 \hat{n} \cdot \vec{S}_2 \hat{n} \cdot \vec{v}_1 \hat{n} \cdot \vec{v}_2 + 10 \vec{S}_1 \cdot \vec{S}_2 \hat{n} \cdot \vec{v}_1 \hat{n} \cdot \vec{v}_2 - \right. \right. \\ \left. \left. 6 \hat{n} \cdot \vec{S}_2 \hat{n} \cdot \vec{v}_2 \vec{S}_1 \cdot \vec{v}_1 + 4 \hat{n} \cdot \vec{S}_2 \hat{n} \cdot \vec{v}_2 \vec{S}_1 \cdot \vec{v}_2 - 6 \hat{n} \cdot \vec{S}_1 \hat{n} \cdot \vec{v}_2 \vec{S}_2 \cdot \vec{v}_1 + 4 \hat{n} \cdot \vec{S}_1 \hat{n} \cdot \vec{v}_2 \vec{S}_2 \cdot \vec{v}_2 - 10 \hat{n} \cdot \vec{S}_2 \hat{n} \cdot \vec{v}_1 \vec{S}_1 \cdot \vec{v}_2 - \right. \right. \\ \left. \left. 10 \hat{n} \cdot \vec{S}_1 \hat{n} \cdot \vec{v}_1 \vec{S}_2 \cdot \vec{v}_2 - 6 \vec{v}_1 \cdot \vec{v}_2 \hat{n} \cdot \vec{S}_1 \hat{n} \cdot \vec{S}_2 + 2 \vec{S}_1 \cdot \vec{v}_2 \vec{S}_2 \cdot \vec{v}_1 + 2 \vec{S}_1 \cdot \vec{v}_1 \vec{S}_2 \cdot \vec{v}_2 - 2 \vec{S}_1 \cdot \vec{S}_2 \vec{v}_1 \cdot \vec{v}_2 \right) + \right. \\ \left. \frac{1}{r^4} \left( 10 \hat{n} \cdot \vec{S}_2 \hat{n} \cdot \vec{S}_1 \hat{n} \cdot \vec{v}_1 + 6 \vec{S}_1 \cdot \vec{S}_2 \hat{n} \cdot \vec{v}_1 - 4 \hat{n} \cdot \vec{S}_2 \hat{n} \cdot \vec{S}_1 \hat{n} \cdot \vec{v}_2 - 6 \hat{n} \cdot \vec{S}_1 \hat{n} \cdot \vec{S}_2 \hat{n} \cdot \vec{v}_2 - 2 \vec{S}_1 \cdot \vec{S}_2 \hat{n} \cdot \vec{v}_2 + \right. \right. \\ \left. \left. 2 \hat{n} \cdot \vec{S}_2 \vec{S}_1 \cdot \vec{v}_2 - 2 \hat{n} \cdot \vec{S}_1 \vec{S}_2 \cdot \vec{v}_1 - 4 \vec{S}_1 \cdot \vec{S}_2 \hat{n} \cdot \vec{v}_2 - 2 \hat{n} \cdot \vec{S}_2 \vec{S}_1 \cdot \vec{v}_1 + 2 \hat{n} \cdot \vec{S}_1 \vec{S}_2 \cdot \vec{v}_2 \right) + \frac{-2 \hat{n} \cdot \vec{S}_1 \hat{n} \cdot \vec{S}_2 - 2 \vec{S}_1 \cdot \vec{S}_2}{r^3} \right\}$$

{DiagS1S2[3, 4, 12],

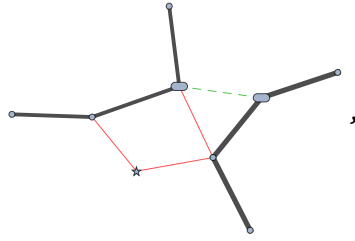

$$G^3 m_1 m_2 \left\{ \frac{1}{r^5} \left( -36 \hat{n} \cdot \vec{S}_1 \hat{n} \cdot \vec{S}_2 (\hat{n} \cdot \vec{v}_2)^2 + 8 \vec{S}_1 \cdot \vec{S}_2 (\hat{n} \cdot \vec{v}_2)^2 + 42 \hat{n} \cdot \vec{S}_1 \hat{n} \cdot \vec{S}_2 \hat{n} \cdot \vec{v}_1 \hat{n} \cdot \vec{v}_2 - 10 \vec{S}_1 \cdot \vec{S}_2 \hat{n} \cdot \vec{v}_1 \hat{n} \cdot \vec{v}_2 - \right. \right. \\ \left. \left. 6 \hat{n} \cdot \vec{S}_2 \hat{n} \cdot \vec{v}_2 \vec{S}_1 \cdot \vec{v}_1 + 6 \hat{n} \cdot \vec{S}_2 \hat{n} \cdot \vec{v}_2 \vec{S}_1 \cdot \vec{v}_2 - 6 \hat{n} \cdot \vec{S}_1 \hat{n} \cdot \vec{v}_2 \vec{S}_2 \cdot \vec{v}_1 + 6 \hat{n} \cdot \vec{S}_1 \hat{n} \cdot \vec{v}_2 \vec{S}_2 \cdot \vec{v}_2 - 6 \vec{v}_1 \cdot \vec{v}_2 \hat{n} \cdot \vec{S}_1 \hat{n} \cdot \vec{S}_2 + \right. \right. \\ \left. \left. 2 \vec{S}_1 \cdot \vec{S}_2 \vec{v}_1 \cdot \vec{v}_2 \right) + \frac{-6 \hat{n} \cdot \vec{S}_2 \hat{n} \cdot \vec{S}_1 \hat{n} \cdot \vec{v}_2 - 6 \hat{n} \cdot \vec{S}_1 \hat{n} \cdot \vec{S}_2 \hat{n} \cdot \vec{v}_2 + 2 \vec{S}_1 \cdot \vec{S}_2 \hat{n} \cdot \vec{v}_2 + 2 \vec{S}_1 \cdot \vec{S}_2 \hat{n} \cdot \vec{v}_2}{r^4} \right\}$$

{DiagS1S2[3, 4, 13],

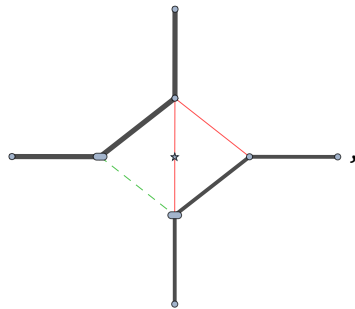

$$G^3 m_1 m_2 \left\{ \frac{1}{r^5} \left( 24 \hat{n} \cdot \vec{S}_1 \hat{n} \cdot \vec{S}_2 (\hat{n} \cdot \vec{v}_2)^2 - 4 \vec{S}_1 \cdot \vec{S}_2 (\hat{n} \cdot \vec{v}_2)^2 - 18 \hat{n} \cdot \vec{S}_1 \hat{n} \cdot \vec{S}_2 \hat{n} \cdot \vec{v}_1 \hat{n} \cdot \vec{v}_2 + 2 \vec{S}_1 \cdot \vec{S}_2 \hat{n} \cdot \vec{v}_1 \hat{n} \cdot \vec{v}_2 + \right. \right. \\ \left. \left. 6 \hat{n} \cdot \vec{S}_2 \hat{n} \cdot \vec{v}_2 \vec{S}_1 \cdot \vec{v}_1 - 6 \hat{n} \cdot \vec{S}_2 \hat{n} \cdot \vec{v}_2 \vec{S}_1 \cdot \vec{v}_2 + 6 \hat{n} \cdot \vec{S}_1 \hat{n} \cdot \vec{v}_2 \vec{S}_2 \cdot \vec{v}_1 - 6 \hat{n} \cdot \vec{S}_1 \hat{n} \cdot \vec{v}_2 \vec{S}_2 \cdot \vec{v}_2 - 6 \vec{v}_1 \cdot \vec{v}_2 \hat{n} \cdot \vec{S}_1 \hat{n} \cdot \vec{S}_2 + \right. \right. \\ \left. \left. 2 \vec{S}_1 \cdot \vec{S}_2 \vec{v}_1 \cdot \vec{v}_2 \right) + \frac{-6 \hat{n} \cdot \vec{S}_2 \hat{n} \cdot \vec{S}_1 \hat{n} \cdot \vec{v}_2 - 6 \hat{n} \cdot \vec{S}_1 \hat{n} \cdot \vec{S}_2 \hat{n} \cdot \vec{v}_2 + 2 \vec{S}_1 \cdot \vec{S}_2 \hat{n} \cdot \vec{v}_2 + 2 \vec{S}_1 \cdot \vec{S}_2 \hat{n} \cdot \vec{v}_2}{r^4} \right\}$$

$$2 \vec{S}_1 \cdot \vec{S}_2 \vec{v}_1 \cdot \vec{v}_2 \Big) + \frac{6 \hat{n} \cdot \vec{S}_2 \hat{n} \cdot \vec{S}_1 \hat{n} \cdot \vec{v}_2 + 6 \hat{n} \cdot \vec{S}_1 \hat{n} \cdot \vec{S}_2 \hat{n} \cdot \vec{v}_2 - 2 \vec{S}_1 \cdot \vec{S}_2 \hat{n} \cdot \vec{v}_2 - 2 \vec{S}_1 \cdot \vec{S}_2 \hat{n} \cdot \vec{v}_2}{r^4} \Bigg\}$$

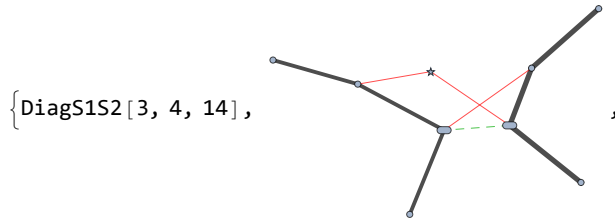

$$G^3 m_1 m_2 \left\{ \frac{1}{r^5} \left( -144 \hat{n} \cdot \vec{S}_1 \hat{n} \cdot \vec{S}_2 (\hat{n} \cdot \vec{v}_2)^2 + 32 \vec{S}_1 \cdot \vec{S}_2 (\hat{n} \cdot \vec{v}_2)^2 + \right. \right. \\ 168 \hat{n} \cdot \vec{S}_1 \hat{n} \cdot \vec{S}_2 \hat{n} \cdot \vec{v}_1 \hat{n} \cdot \vec{v}_2 - 40 \vec{S}_1 \cdot \vec{S}_2 \hat{n} \cdot \vec{v}_1 \hat{n} \cdot \vec{v}_2 - 24 \hat{n} \cdot \vec{S}_2 \hat{n} \cdot \vec{v}_2 \vec{S}_1 \cdot \vec{v}_1 + 24 \hat{n} \cdot \vec{S}_2 \hat{n} \cdot \vec{v}_2 \vec{S}_1 \cdot \vec{v}_2 - \\ 24 \hat{n} \cdot \vec{S}_1 \hat{n} \cdot \vec{v}_2 \vec{S}_2 \cdot \vec{v}_1 + 24 \hat{n} \cdot \vec{S}_1 \hat{n} \cdot \vec{v}_2 \vec{S}_2 \cdot \vec{v}_2 - 24 \vec{v}_1 \cdot \vec{v}_2 \hat{n} \cdot \vec{S}_1 \hat{n} \cdot \vec{S}_2 + 8 \vec{S}_1 \cdot \vec{S}_2 \vec{v}_1 \cdot \vec{v}_2 \Big) + \\ \left. \frac{-24 \hat{n} \cdot \vec{S}_2 \hat{n} \cdot \vec{S}_1 \hat{n} \cdot \vec{v}_2 - 24 \hat{n} \cdot \vec{S}_1 \hat{n} \cdot \vec{S}_2 \hat{n} \cdot \vec{v}_2 + 8 \vec{S}_1 \cdot \vec{S}_2 \hat{n} \cdot \vec{v}_2 + 8 \vec{S}_1 \cdot \vec{S}_2 \hat{n} \cdot \vec{v}_2}{r^4} \right\}$$

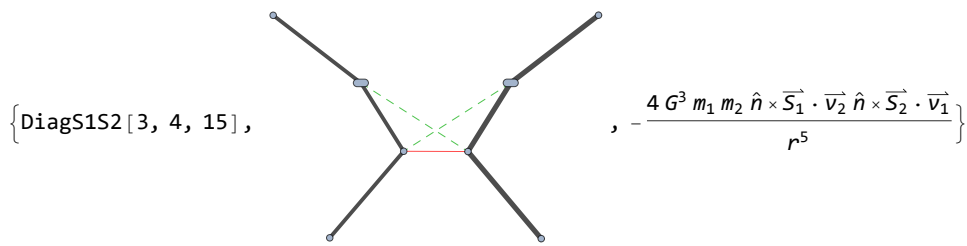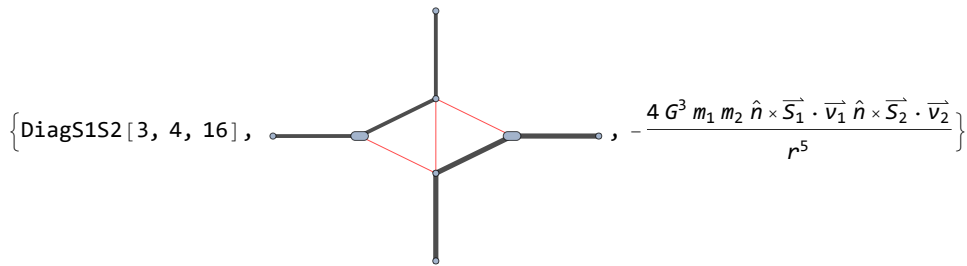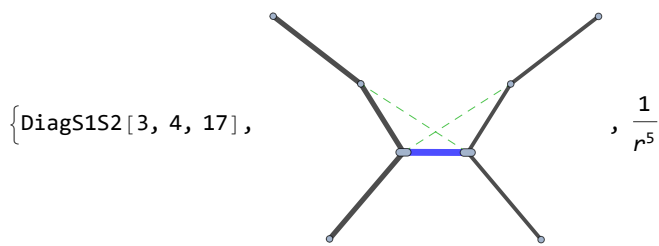

$$G^3 m_1 m_2 \left\{ 28 \hat{n} \times \vec{S}_1 \cdot \vec{v}_2 \hat{n} \times \vec{S}_2 \cdot \vec{v}_1 - 4 \hat{n} \times \vec{S}_1 \cdot \vec{v}_1 \hat{n} \times \vec{S}_2 \cdot \vec{v}_2 + 8 \vec{S}_1 \cdot \vec{S}_2 \hat{n} \cdot \vec{v}_1 \hat{n} \cdot \vec{v}_2 - \right. \\ \left. 4 \hat{n} \cdot \vec{S}_2 \hat{n} \cdot \vec{v}_2 \vec{S}_1 \cdot \vec{v}_1 - 4 \hat{n} \cdot \vec{S}_1 \hat{n} \cdot \vec{v}_1 \vec{S}_2 \cdot \vec{v}_2 + 4 \vec{v}_1 \cdot \vec{v}_2 \hat{n} \cdot \vec{S}_1 \hat{n} \cdot \vec{S}_2 + 4 \vec{S}_1 \cdot \vec{v}_1 \vec{S}_2 \cdot \vec{v}_2 - 8 \vec{S}_1 \cdot \vec{S}_2 \vec{v}_1 \cdot \vec{v}_2 \right\}$$

$\{\text{DiagS1S2}[3, 4, 18],$ 
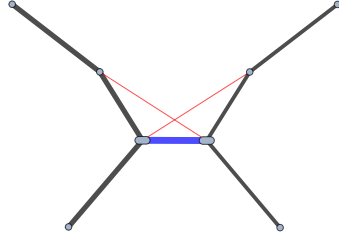
 $, \frac{1}{r^5}$ 

$$G^3 m_1 m_2 \left( -4 \hat{n} \cdot \vec{S}_1 \cdot \vec{v}_2 \hat{n} \times \vec{S}_2 \cdot \vec{v}_1 - 4 \hat{n} \times \vec{S}_1 \cdot \vec{v}_1 \hat{n} \times \vec{S}_2 \cdot \vec{v}_2 - 8 \vec{S}_1 \cdot \vec{S}_2 \hat{n} \cdot \vec{v}_1 \hat{n} \cdot \vec{v}_2 + \right. \\ \left. 4 \hat{n} \cdot \vec{S}_2 \hat{n} \cdot \vec{v}_1 \vec{S}_1 \cdot \vec{v}_2 + 4 \hat{n} \cdot \vec{S}_1 \hat{n} \cdot \vec{v}_2 \vec{S}_2 \cdot \vec{v}_1 + 4 \vec{v}_1 \cdot \vec{v}_2 \hat{n} \cdot \vec{S}_1 \hat{n} \cdot \vec{S}_2 + 4 \vec{S}_1 \cdot \vec{v}_2 \vec{S}_2 \cdot \vec{v}_1 - 8 \vec{S}_1 \cdot \vec{S}_2 \vec{v}_1 \cdot \vec{v}_2 \right) \}$$

 $\{\text{DiagS1S2}[3, 4, 19],$ 
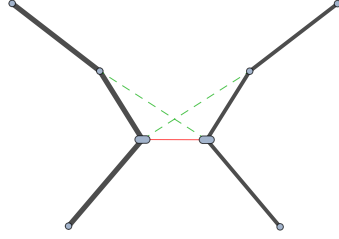
 $, - \frac{64 G^3 m_1 m_2 \hat{n} \times \vec{S}_1 \cdot \vec{v}_2 \hat{n} \times \vec{S}_2 \cdot \vec{v}_1}{r^5} \}$ 
 $\{\text{DiagS1S2}[3, 4, 20],$ 
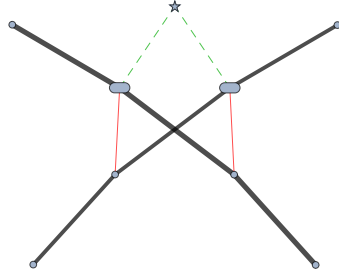
 $,$ 

$$G^3 m_1 m_2 \left( \frac{1}{r^5} \left( -32 \hat{n} \cdot \vec{S}_1 \hat{n} \cdot \vec{S}_2 (\hat{n} \cdot \vec{v}_1)^2 - 16 \vec{S}_1 \cdot \vec{S}_2 (\hat{n} \cdot \vec{v}_1)^2 + 184 \hat{n} \cdot \vec{S}_1 \hat{n} \cdot \vec{S}_2 \hat{n} \cdot \vec{v}_2 \hat{n} \cdot \vec{v}_1 + 56 \vec{S}_1 \cdot \vec{S}_2 \hat{n} \cdot \vec{v}_2 \hat{n} \cdot \vec{v}_1 + \right. \right. \\ \left. \left. 8 \hat{n} \cdot \vec{S}_2 \hat{n} \cdot \vec{v}_1 \vec{S}_1 \cdot \vec{v}_1 - 32 \hat{n} \cdot \vec{S}_2 \hat{n} \cdot \vec{v}_1 \vec{S}_1 \cdot \vec{v}_2 + 8 \hat{n} \cdot \vec{S}_1 \hat{n} \cdot \vec{v}_1 \vec{S}_2 \cdot \vec{v}_1 - 32 \hat{n} \cdot \vec{S}_1 \hat{n} \cdot \vec{v}_1 \vec{S}_2 \cdot \vec{v}_2 - 32 \hat{n} \cdot \vec{S}_1 \hat{n} \cdot \vec{S}_2 \right. \right. \\ \left. \left. (\hat{n} \cdot \vec{v}_2)^2 - 16 \vec{S}_1 \cdot \vec{S}_2 (\hat{n} \cdot \vec{v}_2)^2 - 32 \hat{n} \cdot \vec{S}_2 \hat{n} \cdot \vec{v}_2 \vec{S}_1 \cdot \vec{v}_1 + 8 \hat{n} \cdot \vec{S}_2 \hat{n} \cdot \vec{v}_2 \vec{S}_1 \cdot \vec{v}_2 - 32 \hat{n} \cdot \vec{S}_1 \hat{n} \cdot \vec{v}_2 \vec{S}_2 \cdot \vec{v}_1 + \right. \right. \\ \left. \left. 8 \hat{n} \cdot \vec{S}_1 \hat{n} \cdot \vec{v}_2 \vec{S}_2 \cdot \vec{v}_2 - 24 \vec{v}_1 \cdot \vec{v}_2 \hat{n} \cdot \vec{S}_1 \hat{n} \cdot \vec{S}_2 + 8 \vec{S}_1 \cdot \vec{v}_2 \vec{S}_2 \cdot \vec{v}_1 + 8 \vec{S}_1 \cdot \vec{v}_1 \vec{S}_2 \cdot \vec{v}_2 - 8 \vec{S}_1 \cdot \vec{S}_2 \vec{v}_1 \cdot \vec{v}_2 \right) + \right. \\ \left. \frac{1}{r^4} \left( 32 \hat{n} \cdot \vec{S}_2 \hat{n} \cdot \vec{S}_1 \hat{n} \cdot \vec{v}_1 + 8 \hat{n} \cdot \vec{S}_1 \hat{n} \cdot \vec{S}_2 \hat{n} \cdot \vec{v}_1 + 8 \vec{S}_1 \cdot \vec{S}_2 \hat{n} \cdot \vec{v}_1 + 16 \vec{S}_1 \cdot \vec{S}_2 \hat{n} \cdot \vec{v}_1 - 8 \hat{n} \cdot \vec{S}_2 \hat{n} \cdot \vec{S}_1 \hat{n} \cdot \vec{v}_2 - \right. \right. \\ \left. \left. 32 \hat{n} \cdot \vec{S}_1 \hat{n} \cdot \vec{S}_2 \hat{n} \cdot \vec{v}_2 - 16 \vec{S}_1 \cdot \vec{S}_2 \hat{n} \cdot \vec{v}_2 + 8 \hat{n} \cdot \vec{S}_2 \vec{S}_1 \cdot \vec{v}_2 - 8 \hat{n} \cdot \vec{S}_1 \vec{S}_2 \cdot \vec{v}_1 - \right. \right. \\ \left. \left. 8 \vec{S}_1 \cdot \vec{S}_2 \hat{n} \cdot \vec{v}_2 - 8 \hat{n} \cdot \vec{S}_2 \vec{S}_1 \cdot \vec{v}_1 + 8 \hat{n} \cdot \vec{S}_1 \vec{S}_2 \cdot \vec{v}_2 \right) + \frac{-8 \hat{n} \cdot \vec{S}_1 \hat{n} \cdot \vec{S}_2 - 8 \vec{S}_1 \cdot \vec{S}_2}{r^3} \right) \}$$

 $\{\text{DiagS1S2}[3, 4, 21],$ 
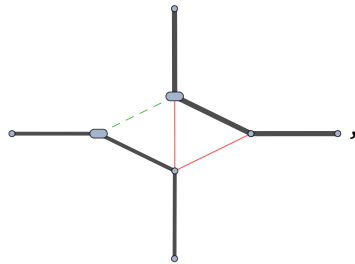
 $,$

$$G^3 m_1 m_2 \left( \frac{8 \vec{S}_1 \cdot \vec{a}_2 \hat{n} \cdot \vec{S}_2 - 8 \vec{S}_1 \cdot \vec{S}_2 \hat{n} \cdot \vec{a}_2 - 8 \vec{S}_1 \cdot \vec{S}_2 \hat{n} \cdot \vec{v}_2 + 8 \hat{n} \cdot \vec{S}_2 \vec{S}_1 \cdot \vec{v}_2}{r^4} + \frac{1}{r^5} \right. \\ \left. \left( 18 \hat{n} \times \vec{S}_1 \cdot \vec{v}_2 \hat{n} \times \vec{S}_2 \cdot \vec{v}_2 + 4 \vec{S}_1 \cdot \vec{S}_2 (\hat{n} \cdot \vec{v}_1)^2 - 8 \vec{S}_1 \cdot \vec{S}_2 \hat{n} \cdot \vec{v}_2 \hat{n} \cdot \vec{v}_1 - 4 \hat{n} \cdot \vec{S}_1 \hat{n} \cdot \vec{v}_1 \vec{S}_2 \cdot \vec{v}_1 - \right. \right. \\ \left. \left. 6 \vec{S}_1 \cdot \vec{S}_2 (\hat{n} \cdot \vec{v}_2)^2 + 6 \hat{n} \cdot \vec{S}_2 \hat{n} \cdot \vec{v}_2 \vec{S}_1 \cdot \vec{v}_2 + 8 \hat{n} \cdot \vec{S}_1 \hat{n} \cdot \vec{v}_2 \vec{S}_2 \cdot \vec{v}_1 - 18 \vec{v}_1 \cdot \vec{v}_1 \hat{n} \cdot \vec{S}_1 \hat{n} \cdot \vec{S}_2 + \right. \right. \\ \left. \left. 54 \vec{v}_2 \cdot \vec{v}_2 \hat{n} \cdot \vec{S}_1 \hat{n} \cdot \vec{S}_2 + 4 \vec{S}_1 \cdot \vec{v}_2 \vec{S}_2 \cdot \vec{v}_2 + 6 \vec{S}_1 \cdot \vec{S}_2 \vec{v}_1 \cdot \vec{v}_1 - 22 \vec{S}_1 \cdot \vec{S}_2 \vec{v}_2 \cdot \vec{v}_2 \right) \right) \Bigg\}$$

{DiagS1S2 [3, 4, 22],

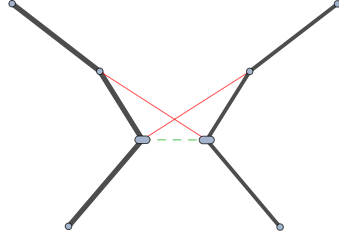

,  $\frac{1}{r^5}$

$$G^3 m_1 m_2 \left( -32 \vec{S}_1 \cdot \vec{S}_2 \hat{n} \cdot \vec{v}_1 \hat{n} \cdot \vec{v}_2 + 16 \hat{n} \cdot \vec{S}_2 \hat{n} \cdot \vec{v}_1 \vec{S}_1 \cdot \vec{v}_2 + 16 \hat{n} \cdot \vec{S}_1 \hat{n} \cdot \vec{v}_2 \vec{S}_2 \cdot \vec{v}_1 - \right. \\ \left. 72 \vec{v}_1 \cdot \vec{v}_1 \hat{n} \cdot \vec{S}_1 \hat{n} \cdot \vec{S}_2 - 72 \vec{v}_2 \cdot \vec{v}_2 \hat{n} \cdot \vec{S}_1 \hat{n} \cdot \vec{S}_2 + 24 \vec{S}_1 \cdot \vec{S}_2 \vec{v}_1 \cdot \vec{v}_1 + 24 \vec{S}_1 \cdot \vec{S}_2 \vec{v}_2 \cdot \vec{v}_2 \right) \Bigg\}$$

{DiagS1S2 [3, 5, 1],

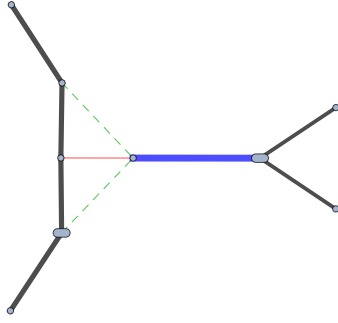

,  $\frac{1}{r^5}$

$$G^3 m_1^2 \left( 8 \hat{n} \times \vec{S}_1 \cdot \vec{v}_2 \hat{n} \times \vec{S}_2 \cdot \vec{v}_1 - \frac{64}{7} \hat{n} \times \vec{S}_1 \cdot \vec{v}_1 \hat{n} \times \vec{S}_2 \cdot \vec{v}_2 + \frac{64}{7} \vec{S}_1 \cdot \vec{S}_2 \hat{n} \cdot \vec{v}_1 \hat{n} \cdot \vec{v}_2 - \right. \\ \left. \frac{64}{7} \hat{n} \cdot \vec{S}_1 \hat{n} \cdot \vec{v}_2 \vec{S}_2 \cdot \vec{v}_1 - 8 \vec{v}_1 \cdot \vec{v}_2 \hat{n} \cdot \vec{S}_1 \hat{n} \cdot \vec{S}_2 + \frac{8}{5} \vec{S}_1 \cdot \vec{v}_1 \vec{S}_2 \cdot \vec{v}_2 + \frac{16}{5} \vec{S}_1 \cdot \vec{S}_2 \vec{v}_1 \cdot \vec{v}_2 \right) \Bigg\}$$

{DiagS1S2 [3, 5, 2],

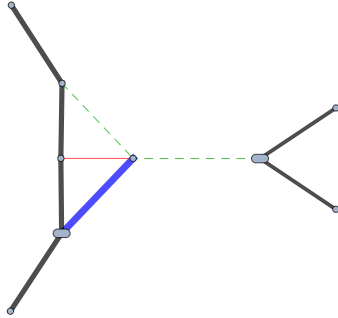

,  $\frac{1}{r^5}$

$$G^3 m_1^2 \left( 40 \hat{n} \times \vec{S}_1 \cdot \vec{v}_1 \hat{n} \times \vec{S}_2 \cdot \vec{v}_1 + 8 \vec{S}_1 \cdot \vec{S}_2 (\hat{n} \cdot \vec{v}_1)^2 - 8 \hat{n} \cdot \vec{S}_1 \hat{n} \cdot \vec{v}_1 \vec{S}_2 \cdot \vec{v}_1 + \right. \\ \left. 32 \vec{v}_1 \cdot \vec{v}_1 \hat{n} \cdot \vec{S}_1 \hat{n} \cdot \vec{S}_2 + \frac{48}{5} \vec{S}_1 \cdot \vec{v}_1 \vec{S}_2 \cdot \vec{v}_1 - \frac{144}{5} \vec{S}_1 \cdot \vec{S}_2 \vec{v}_1 \cdot \vec{v}_1 \right) \Bigg\}$$

$\{\text{DiagS1S2}[3, 5, 3],$

$$\begin{aligned} G^3 m_1^2 \left( \frac{1}{r^5 \in_d} \left( 168 \hat{n} \cdot \vec{S}_1 \hat{n} \cdot \vec{S}_2 \left( \hat{n} \cdot \vec{v}_1 \right)^2 - 24 \vec{S}_1 \cdot \vec{S}_2 \left( \hat{n} \cdot \vec{v}_1 \right)^2 - 48 \hat{n} \cdot \vec{S}_2 \hat{n} \cdot \vec{v}_1 \vec{S}_1 \cdot \vec{v}_1 - \right. \right. \\ \left. \left. 48 \hat{n} \cdot \vec{S}_1 \hat{n} \cdot \vec{v}_1 \vec{S}_2 \cdot \vec{v}_1 - 24 \vec{v}_1 \cdot \vec{v}_1 \hat{n} \cdot \vec{S}_1 \hat{n} \cdot \vec{S}_2 + \frac{48}{5} \vec{S}_1 \cdot \vec{v}_1 \vec{S}_2 \cdot \vec{v}_1 + \frac{24}{5} \vec{S}_1 \cdot \vec{S}_2 \vec{v}_1 \cdot \vec{v}_1 \right) + \right. \\ \left. \frac{1}{r^5} \log \left( \frac{r}{R_\theta} \right) \left( -504 \hat{n} \cdot \vec{S}_1 \hat{n} \cdot \vec{S}_2 \left( \hat{n} \cdot \vec{v}_1 \right)^2 + 72 \vec{S}_1 \cdot \vec{S}_2 \left( \hat{n} \cdot \vec{v}_1 \right)^2 + 144 \hat{n} \cdot \vec{S}_2 \hat{n} \cdot \vec{v}_1 \vec{S}_1 \cdot \vec{v}_1 + \right. \right. \\ \left. \left. 144 \hat{n} \cdot \vec{S}_1 \hat{n} \cdot \vec{v}_1 \vec{S}_2 \cdot \vec{v}_1 + 72 \vec{v}_1 \cdot \vec{v}_1 \hat{n} \cdot \vec{S}_1 \hat{n} \cdot \vec{S}_2 - \frac{144}{5} \vec{S}_1 \cdot \vec{v}_1 \vec{S}_2 \cdot \vec{v}_1 - \frac{72}{5} \vec{S}_1 \cdot \vec{S}_2 \vec{v}_1 \cdot \vec{v}_1 \right) + \frac{1}{r^5} \right. \\ \left. \left( -16 \hat{n} \times \vec{S}_1 \cdot \vec{v}_1 \hat{n} \times \vec{S}_2 \cdot \vec{v}_1 + 296 \hat{n} \cdot \vec{S}_1 \hat{n} \cdot \vec{S}_2 \left( \hat{n} \cdot \vec{v}_1 \right)^2 - 72 \vec{S}_1 \cdot \vec{S}_2 \left( \hat{n} \cdot \vec{v}_1 \right)^2 - 64 \hat{n} \cdot \vec{S}_2 \hat{n} \cdot \vec{v}_1 \vec{S}_1 \cdot \vec{v}_1 - \right. \right. \\ \left. \left. 96 \hat{n} \cdot \vec{S}_1 \hat{n} \cdot \vec{v}_1 \vec{S}_2 \cdot \vec{v}_1 - 48 \vec{v}_1 \cdot \vec{v}_1 \hat{n} \cdot \vec{S}_1 \hat{n} \cdot \vec{S}_2 + \frac{256}{25} \vec{S}_1 \cdot \vec{v}_1 \vec{S}_2 \cdot \vec{v}_1 + \frac{608}{25} \vec{S}_1 \cdot \vec{S}_2 \vec{v}_1 \cdot \vec{v}_1 \right) \right) \Bigg\} \end{aligned}$$

$\{\text{DiagS1S2}[3, 5, 4],$

$$\begin{aligned} G^3 m_1^2 & \left( \frac{1}{r^4} \left( -32 \hat{n} \cdot \vec{a}_1 \hat{n} \cdot \vec{S}_1 \hat{n} \cdot \vec{S}_2 + 48 \hat{n} \cdot \vec{S}_1 \hat{n} \cdot \vec{v}_1 \hat{n} \cdot \vec{S}_2 - \frac{144}{25} \vec{S}_1 \cdot \vec{v}_1 \hat{n} \cdot \vec{S}_2 + \right. \right. \\ & \frac{112}{25} \vec{S}_1 \cdot \vec{a}_1 \hat{n} \cdot \vec{S}_2 - 48 \hat{n} \cdot \vec{S}_2 \hat{n} \cdot \vec{S}_1 \hat{n} \cdot \vec{v}_1 - \frac{624}{25} \hat{n} \cdot \vec{v}_1 \vec{S}_1 \cdot \vec{S}_2 + \frac{224}{25} \hat{n} \cdot \vec{S}_1 \vec{S}_2 \cdot \vec{v}_1 + \frac{544}{25} \hat{n} \cdot \vec{v}_1 \vec{S}_1 \cdot \vec{S}_2 + \\ & \left. \frac{512}{25} \hat{n} \cdot \vec{a}_1 \vec{S}_1 \cdot \vec{S}_2 + \frac{144}{25} \hat{n} \cdot \vec{S}_2 \vec{S}_1 \cdot \vec{v}_1 - \frac{48}{25} \hat{n} \cdot \vec{S}_1 \vec{S}_2 \cdot \vec{a}_1 - \frac{144}{25} \hat{n} \cdot \vec{S}_1 \vec{S}_2 \cdot \vec{v}_1 \right) + \frac{1}{r^5} \\ & \left( -160 \hat{n} \cdot \vec{S}_1 \hat{n} \cdot \vec{S}_2 (\hat{n} \cdot \vec{v}_1)^2 + \frac{272}{7} \vec{S}_1 \cdot \vec{S}_2 (\hat{n} \cdot \vec{v}_1)^2 - 432 \hat{n} \cdot \vec{S}_1 \hat{n} \cdot \vec{S}_2 \hat{n} \cdot \vec{v}_2 \hat{n} \cdot \vec{v}_1 + 128 \hat{n} \cdot \vec{v}_2 \vec{S}_1 \cdot \vec{S}_2 \hat{n} \cdot \vec{v}_1 + \right. \\ & 32 \hat{n} \cdot \vec{S}_2 \vec{S}_1 \cdot \vec{v}_1 \hat{n} \cdot \vec{v}_1 + 48 \hat{n} \cdot \vec{S}_2 \vec{S}_1 \cdot \vec{v}_2 \hat{n} \cdot \vec{v}_1 + \frac{400}{7} \hat{n} \cdot \vec{S}_1 \vec{S}_2 \cdot \vec{v}_1 \hat{n} \cdot \vec{v}_1 + 48 \hat{n} \cdot \vec{S}_1 \vec{S}_2 \cdot \vec{v}_2 \hat{n} \cdot \vec{v}_1 - \\ & \frac{160}{7} \hat{n} \times \vec{S}_1 \cdot \vec{v}_1 \hat{n} \times \vec{S}_2 \cdot \vec{v}_1 + 48 \hat{n} \cdot \vec{S}_2 \hat{n} \cdot \vec{v}_2 \vec{S}_1 \cdot \vec{v}_1 + 64 \hat{n} \cdot \vec{S}_1 \hat{n} \cdot \vec{v}_2 \vec{S}_2 \cdot \vec{v}_1 - \frac{304}{25} \vec{S}_1 \cdot \vec{v}_1 \vec{S}_2 \cdot \vec{v}_1 - \frac{224}{25} \vec{S}_1 \cdot \vec{v}_2 \vec{S}_2 \cdot \vec{v}_1 - \\ & \left. \frac{144}{25} \vec{S}_1 \cdot \vec{v}_1 \vec{S}_2 \cdot \vec{v}_2 + 16 \hat{n} \cdot \vec{S}_1 \hat{n} \cdot \vec{S}_2 \vec{v}_1 \cdot \vec{v}_1 - \frac{32}{25} \vec{S}_1 \cdot \vec{S}_2 \vec{v}_1 \cdot \vec{v}_1 + 48 \hat{n} \cdot \vec{S}_1 \hat{n} \cdot \vec{S}_2 \vec{v}_1 \cdot \vec{v}_2 - \frac{544}{25} \vec{S}_1 \cdot \vec{S}_2 \vec{v}_1 \cdot \vec{v}_2 \right) + \\ & \left( \frac{1}{r^4} \left( 48 \hat{n} \cdot \vec{a}_1 \hat{n} \cdot \vec{S}_1 \hat{n} \cdot \vec{S}_2 - 96 \hat{n} \cdot \vec{S}_1 \hat{n} \cdot \vec{v}_1 \hat{n} \cdot \vec{S}_2 + \frac{96}{5} \vec{S}_1 \cdot \vec{v}_1 \hat{n} \cdot \vec{S}_2 - \frac{48}{5} \vec{S}_1 \cdot \vec{a}_1 \hat{n} \cdot \vec{S}_2 + 96 \hat{n} \cdot \vec{S}_2 \hat{n} \cdot \vec{S}_1 \hat{n} \cdot \vec{v}_1 + \right. \right. \\ & \frac{96}{5} \hat{n} \cdot \vec{v}_1 \vec{S}_1 \cdot \vec{S}_2 - \frac{96}{5} \hat{n} \cdot \vec{S}_1 \vec{S}_2 \cdot \vec{v}_1 - \frac{96}{5} \hat{n} \cdot \vec{v}_1 \vec{S}_1 \cdot \vec{S}_2 - \frac{48}{5} \hat{n} \cdot \vec{a}_1 \vec{S}_1 \cdot \vec{S}_2 - \frac{96}{5} \hat{n} \cdot \vec{S}_2 \vec{S}_1 \cdot \vec{v}_1 - \frac{48}{5} \hat{n} \cdot \vec{S}_1 \vec{S}_2 \cdot \vec{a}_1 + \\ & \left. \frac{96}{5} \hat{n} \cdot \vec{S}_1 \vec{S}_2 \cdot \vec{v}_1 \right) + \frac{1}{r^5} \left( 336 \hat{n} \cdot \vec{S}_1 \hat{n} \cdot \vec{S}_2 (\hat{n} \cdot \vec{v}_1)^2 - 48 \vec{S}_1 \cdot \vec{S}_2 (\hat{n} \cdot \vec{v}_1)^2 + 672 \hat{n} \cdot \vec{S}_1 \hat{n} \cdot \vec{S}_2 \hat{n} \cdot \vec{v}_2 \hat{n} \cdot \vec{v}_1 - \right. \end{aligned}$$

$$\begin{aligned}
& 96 \hat{n} \cdot \vec{v}_2 \vec{S}_1 \cdot \vec{S}_2 \hat{n} \cdot \vec{v}_1 - 96 \hat{n} \cdot \vec{S}_2 \vec{S}_1 \cdot \vec{v}_1 \hat{n} \cdot \vec{v}_1 - 96 \hat{n} \cdot \vec{S}_2 \vec{S}_1 \cdot \vec{v}_2 \hat{n} \cdot \vec{v}_1 - 96 \hat{n} \cdot \vec{S}_1 \vec{S}_2 \cdot \vec{v}_1 \hat{n} \cdot \vec{v}_1 - \\
& 96 \hat{n} \cdot \vec{S}_1 \vec{S}_2 \cdot \vec{v}_2 \hat{n} \cdot \vec{v}_1 - 96 \hat{n} \cdot \vec{S}_2 \hat{n} \cdot \vec{v}_2 \vec{S}_1 \cdot \vec{v}_1 - 96 \hat{n} \cdot \vec{S}_1 \hat{n} \cdot \vec{v}_2 \vec{S}_2 \cdot \vec{v}_1 + \frac{96}{5} \vec{S}_1 \cdot \vec{v}_1 \vec{S}_2 \cdot \vec{v}_1 + \frac{96}{5} \vec{S}_1 \cdot \vec{v}_2 \vec{S}_2 \cdot \vec{v}_1 + \\
& \frac{96}{5} \vec{S}_1 \cdot \vec{v}_1 \vec{S}_2 \cdot \vec{v}_2 - 48 \hat{n} \cdot \vec{S}_1 \hat{n} \cdot \vec{S}_2 \vec{v}_1 \cdot \vec{v}_1 + \frac{48}{5} \vec{S}_1 \cdot \vec{S}_2 \vec{v}_1 \cdot \vec{v}_1 - 96 \hat{n} \cdot \vec{S}_1 \hat{n} \cdot \vec{S}_2 \vec{v}_1 \cdot \vec{v}_2 + \frac{96}{5} \vec{S}_1 \cdot \vec{S}_2 \vec{v}_1 \cdot \vec{v}_2 \Big) \Big) \\
& \log \left( \frac{r}{R_\theta} \right) + \frac{1}{\epsilon_d} \left( \frac{1}{r^4} \left( -16 \hat{n} \cdot \vec{a}_1 \hat{n} \cdot \vec{S}_1 \hat{n} \cdot \vec{S}_2 + 32 \hat{n} \cdot \vec{S}_1 \hat{n} \cdot \vec{v}_1 \hat{n} \cdot \vec{S}_2 - \frac{32}{5} \vec{S}_1 \cdot \vec{v}_1 \hat{n} \cdot \vec{S}_2 + \frac{16}{5} \vec{S}_1 \cdot \vec{a}_1 \hat{n} \cdot \vec{S}_2 - \right. \right. \\
& 32 \hat{n} \cdot \vec{S}_2 \hat{n} \cdot \vec{S}_1 \hat{n} \cdot \vec{v}_1 - \frac{32}{5} \hat{n} \cdot \vec{v}_1 \vec{S}_1 \cdot \vec{S}_2 + \frac{32}{5} \hat{n} \cdot \vec{S}_1 \vec{S}_2 \cdot \vec{v}_1 + \frac{32}{5} \hat{n} \cdot \vec{v}_1 \vec{S}_1 \cdot \vec{S}_2 + \\
& \left. \frac{16}{5} \hat{n} \cdot \vec{a}_1 \vec{S}_1 \cdot \vec{S}_2 + \frac{32}{5} \hat{n} \cdot \vec{S}_2 \vec{S}_1 \cdot \vec{v}_1 + \frac{16}{5} \hat{n} \cdot \vec{S}_1 \vec{S}_2 \cdot \vec{a}_1 - \frac{32}{5} \hat{n} \cdot \vec{S}_1 \vec{S}_2 \cdot \vec{v}_1 \right) + \frac{1}{r^5} \\
& \left( -112 \hat{n} \cdot \vec{S}_1 \hat{n} \cdot \vec{S}_2 (\hat{n} \cdot \vec{v}_1)^2 + 16 \vec{S}_1 \cdot \vec{S}_2 (\hat{n} \cdot \vec{v}_1)^2 - 224 \hat{n} \cdot \vec{S}_1 \hat{n} \cdot \vec{S}_2 \hat{n} \cdot \vec{v}_2 \hat{n} \cdot \vec{v}_1 + 32 \hat{n} \cdot \vec{v}_2 \vec{S}_1 \cdot \vec{S}_2 \hat{n} \cdot \vec{v}_1 + \right. \\
& 32 \hat{n} \cdot \vec{S}_2 \vec{S}_1 \cdot \vec{v}_1 \hat{n} \cdot \vec{v}_1 + 32 \hat{n} \cdot \vec{S}_2 \vec{S}_1 \cdot \vec{v}_2 \hat{n} \cdot \vec{v}_1 + 32 \hat{n} \cdot \vec{S}_1 \vec{S}_2 \cdot \vec{v}_1 \hat{n} \cdot \vec{v}_1 + 32 \hat{n} \cdot \vec{S}_1 \vec{S}_2 \cdot \vec{v}_2 \hat{n} \cdot \vec{v}_1 + \\
& 32 \hat{n} \cdot \vec{S}_2 \hat{n} \cdot \vec{v}_2 \vec{S}_1 \cdot \vec{v}_1 + 32 \hat{n} \cdot \vec{S}_1 \hat{n} \cdot \vec{v}_2 \vec{S}_2 \cdot \vec{v}_1 - \frac{32}{5} \vec{S}_1 \cdot \vec{v}_1 \vec{S}_2 \cdot \vec{v}_1 - \frac{32}{5} \vec{S}_1 \cdot \vec{v}_2 \vec{S}_2 \cdot \vec{v}_1 - \frac{32}{5} \vec{S}_1 \cdot \vec{v}_1 \vec{S}_2 \cdot \vec{v}_2 + \\
& \left. \left. 16 \hat{n} \cdot \vec{S}_1 \hat{n} \cdot \vec{S}_2 \vec{v}_1 \cdot \vec{v}_1 - \frac{16}{5} \vec{S}_1 \cdot \vec{S}_2 \vec{v}_1 \cdot \vec{v}_1 + 32 \hat{n} \cdot \vec{S}_1 \hat{n} \cdot \vec{S}_2 \vec{v}_1 \cdot \vec{v}_2 - \frac{32}{5} \vec{S}_1 \cdot \vec{S}_2 \vec{v}_1 \cdot \vec{v}_2 \right) \right) \Big) \Big) \Big\}
\end{aligned}$$

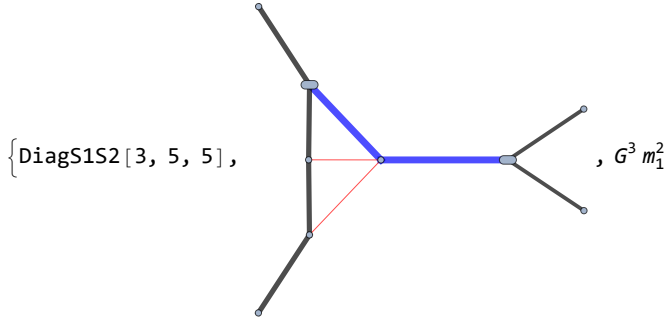

$$\begin{aligned}
& \left( \frac{1}{r^5 \epsilon_d} \left( 2 \hat{n} \cdot \vec{S}_1 \hat{n} \cdot \vec{S}_2 \hat{n} \cdot \vec{v}_1 \hat{n} \cdot \vec{v}_2 - \frac{2}{7} \hat{n} \cdot \vec{v}_1 \vec{S}_1 \cdot \vec{S}_2 \hat{n} \cdot \vec{v}_2 - \frac{2}{7} \hat{n} \cdot \vec{S}_2 \vec{S}_1 \cdot \vec{v}_1 \hat{n} \cdot \vec{v}_2 - \frac{2}{7} \hat{n} \cdot \vec{S}_1 \vec{S}_2 \cdot \vec{v}_1 \hat{n} \cdot \vec{v}_2 - \frac{2}{7} \hat{n} \cdot \vec{S}_2 \hat{n} \cdot \vec{v}_1 \right. \right. \\
& \left. \left. \vec{S}_1 \cdot \vec{v}_2 + \frac{2}{35} \vec{S}_1 \cdot \vec{v}_2 \vec{S}_2 \cdot \vec{v}_1 - \frac{2}{7} \hat{n} \cdot \vec{S}_1 \hat{n} \cdot \vec{v}_1 \vec{S}_2 \cdot \vec{v}_2 + \frac{2}{35} \vec{S}_1 \cdot \vec{v}_1 \vec{S}_2 \cdot \vec{v}_2 - \frac{2}{7} \hat{n} \cdot \vec{S}_1 \hat{n} \cdot \vec{S}_2 \vec{v}_1 \cdot \vec{v}_2 + \frac{2}{35} \vec{S}_1 \cdot \vec{S}_2 \vec{v}_1 \cdot \vec{v}_2 \right) + \right. \\
& \frac{1}{r^5} \left( \frac{5}{7} \hat{n} \times \vec{S}_1 \cdot \vec{v}_2 \hat{n} \times \vec{S}_2 \cdot \vec{v}_1 - \frac{10}{7} \hat{n} \times \vec{S}_1 \cdot \vec{v}_1 \hat{n} \times \vec{S}_2 \cdot \vec{v}_2 + 7 \hat{n} \cdot \vec{S}_1 \hat{n} \cdot \vec{S}_2 \hat{n} \cdot \vec{v}_1 \hat{n} \cdot \vec{v}_2 - \frac{127}{49} \hat{n} \cdot \vec{v}_1 \hat{n} \cdot \vec{v}_2 \vec{S}_1 \cdot \vec{S}_2 - \right. \\
& \frac{43}{49} \hat{n} \cdot \vec{S}_2 \hat{n} \cdot \vec{v}_2 \vec{S}_1 \cdot \vec{v}_1 - \frac{43}{49} \hat{n} \cdot \vec{S}_2 \hat{n} \cdot \vec{v}_1 \vec{S}_1 \cdot \vec{v}_2 - \frac{1}{49} \hat{n} \cdot \vec{S}_1 \hat{n} \cdot \vec{v}_2 \vec{S}_2 \cdot \vec{v}_1 - \frac{387 \vec{S}_1 \cdot \vec{v}_2 \vec{S}_2 \cdot \vec{v}_1}{1225} - \\
& \left. \frac{43}{49} \hat{n} \cdot \vec{S}_1 \hat{n} \cdot \vec{v}_1 \vec{S}_2 \cdot \vec{v}_2 + \frac{348 \vec{S}_1 \cdot \vec{v}_1 \vec{S}_2 \cdot \vec{v}_2}{1225} - \frac{78}{49} \hat{n} \cdot \vec{S}_1 \hat{n} \cdot \vec{S}_2 \vec{v}_1 \cdot \vec{v}_2 + \frac{1293 \vec{S}_1 \cdot \vec{S}_2 \vec{v}_1 \cdot \vec{v}_2}{1225} \right) + \frac{1}{r^5} \\
& \left( -6 \hat{n} \cdot \vec{S}_1 \hat{n} \cdot \vec{S}_2 \hat{n} \cdot \vec{v}_1 \hat{n} \cdot \vec{v}_2 + \frac{6}{7} \hat{n} \cdot \vec{v}_1 \vec{S}_1 \cdot \vec{S}_2 \hat{n} \cdot \vec{v}_2 + \frac{6}{7} \hat{n} \cdot \vec{S}_2 \vec{S}_1 \cdot \vec{v}_1 \hat{n} \cdot \vec{v}_2 + \frac{6}{7} \hat{n} \cdot \vec{S}_1 \vec{S}_2 \cdot \vec{v}_1 \hat{n} \cdot \vec{v}_2 + \right. \\
& \frac{6}{7} \hat{n} \cdot \vec{S}_2 \hat{n} \cdot \vec{v}_1 \vec{S}_1 \cdot \vec{v}_2 - \frac{6}{35} \vec{S}_1 \cdot \vec{v}_2 \vec{S}_2 \cdot \vec{v}_1 + \frac{6}{7} \hat{n} \cdot \vec{S}_1 \hat{n} \cdot \vec{v}_1 \vec{S}_2 \cdot \vec{v}_2 - \\
& \left. \frac{6}{35} \vec{S}_1 \cdot \vec{v}_1 \vec{S}_2 \cdot \vec{v}_2 + \frac{6}{7} \hat{n} \cdot \vec{S}_1 \hat{n} \cdot \vec{S}_2 \vec{v}_1 \cdot \vec{v}_2 - \frac{6}{35} \vec{S}_1 \cdot \vec{S}_2 \vec{v}_1 \cdot \vec{v}_2 \right) \log \left( \frac{r}{R_\theta} \right) \Big) \Big\}
\end{aligned}$$



{DiagS1S2 [3, 5, 6],

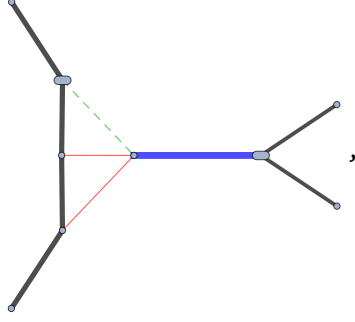

$$G^3 m_1^2 \left( \frac{1}{r^5} \left( \frac{2}{7} \hat{n} \cdot \vec{S}_1 \cdot \vec{v}_2 \hat{n} \cdot \vec{S}_2 \cdot \vec{v}_1 - 7 \hat{n} \cdot \vec{S}_1 \hat{n} \cdot \vec{S}_2 \hat{n} \cdot \vec{v}_1 \hat{n} \cdot \vec{v}_2 + \frac{99}{49} \hat{n} \cdot \vec{v}_1 \hat{n} \cdot \vec{v}_2 \vec{S}_1 \cdot \vec{S}_2 + \right. \right. \\ \left. \frac{43}{49} \hat{n} \cdot \vec{S}_2 \hat{n} \cdot \vec{v}_2 \vec{S}_1 \cdot \vec{v}_1 + \frac{43}{49} \hat{n} \cdot \vec{S}_2 \hat{n} \cdot \vec{v}_1 \vec{S}_1 \cdot \vec{v}_2 + \frac{29}{49} \hat{n} \cdot \vec{S}_1 \hat{n} \cdot \vec{v}_2 \vec{S}_2 \cdot \vec{v}_1 - \frac{103 \vec{S}_1 \cdot \vec{v}_2 \vec{S}_2 \cdot \vec{v}_1}{1225} + \right. \\ \left. \frac{43}{49} \hat{n} \cdot \vec{S}_1 \hat{n} \cdot \vec{v}_1 \vec{S}_2 \cdot \vec{v}_2 - \frac{103 \vec{S}_1 \cdot \vec{v}_1 \vec{S}_2 \cdot \vec{v}_2}{1225} + \frac{29}{49} \hat{n} \cdot \vec{S}_1 \hat{n} \cdot \vec{S}_2 \vec{v}_1 \cdot \vec{v}_2 - \frac{313 \vec{S}_1 \cdot \vec{S}_2 \vec{v}_1 \cdot \vec{v}_2}{1225} \right) + \frac{1}{r^5} \\ \left( 6 \hat{n} \cdot \vec{S}_1 \hat{n} \cdot \vec{S}_2 \hat{n} \cdot \vec{v}_1 \hat{n} \cdot \vec{v}_2 - \frac{6}{7} \hat{n} \cdot \vec{v}_1 \vec{S}_1 \cdot \vec{S}_2 \hat{n} \cdot \vec{v}_2 - \frac{6}{7} \hat{n} \cdot \vec{S}_2 \vec{S}_1 \cdot \vec{v}_1 \hat{n} \cdot \vec{v}_2 - \frac{6}{7} \hat{n} \cdot \vec{S}_1 \vec{S}_2 \cdot \vec{v}_1 \hat{n} \cdot \vec{v}_2 - \frac{6}{7} \hat{n} \cdot \vec{S}_2 \hat{n} \cdot \vec{v}_1 \right. \\ \left. \vec{S}_1 \cdot \vec{v}_2 + \frac{6}{35} \vec{S}_1 \cdot \vec{v}_2 \vec{S}_2 \cdot \vec{v}_1 - \frac{6}{7} \hat{n} \cdot \vec{S}_1 \hat{n} \cdot \vec{v}_1 \vec{S}_2 \cdot \vec{v}_2 + \frac{6}{35} \vec{S}_1 \cdot \vec{v}_1 \vec{S}_2 \cdot \vec{v}_2 - \frac{6}{7} \hat{n} \cdot \vec{S}_1 \hat{n} \cdot \vec{S}_2 \vec{v}_1 \cdot \vec{v}_2 + \frac{6}{35} \vec{S}_1 \cdot \vec{S}_2 \vec{v}_1 \cdot \vec{v}_2 \right) \\ \log \left( \frac{r}{R_0} \right) + \frac{1}{r^5 \epsilon_d} \left( -2 \hat{n} \cdot \vec{S}_1 \hat{n} \cdot \vec{S}_2 \hat{n} \cdot \vec{v}_1 \hat{n} \cdot \vec{v}_2 + \frac{2}{7} \hat{n} \cdot \vec{v}_1 \vec{S}_1 \cdot \vec{S}_2 \hat{n} \cdot \vec{v}_2 + \frac{2}{7} \hat{n} \cdot \vec{S}_2 \vec{S}_1 \cdot \vec{v}_1 \hat{n} \cdot \vec{v}_2 + \right. \\ \left. \frac{2}{7} \hat{n} \cdot \vec{S}_1 \vec{S}_2 \cdot \vec{v}_1 \hat{n} \cdot \vec{v}_2 + \frac{2}{7} \hat{n} \cdot \vec{S}_2 \hat{n} \cdot \vec{v}_1 \vec{S}_1 \cdot \vec{v}_2 - \frac{2}{35} \vec{S}_1 \cdot \vec{v}_2 \vec{S}_2 \cdot \vec{v}_1 + \right. \\ \left. \frac{2}{7} \hat{n} \cdot \vec{S}_1 \hat{n} \cdot \vec{v}_1 \vec{S}_2 \cdot \vec{v}_2 - \frac{2}{35} \vec{S}_1 \cdot \vec{v}_1 \vec{S}_2 \cdot \vec{v}_2 + \frac{2}{7} \hat{n} \cdot \vec{S}_1 \hat{n} \cdot \vec{S}_2 \vec{v}_1 \cdot \vec{v}_2 - \frac{2}{35} \vec{S}_1 \cdot \vec{S}_2 \vec{v}_1 \cdot \vec{v}_2 \right) \Bigg\}$$

{DiagS1S2 [3, 5, 7],

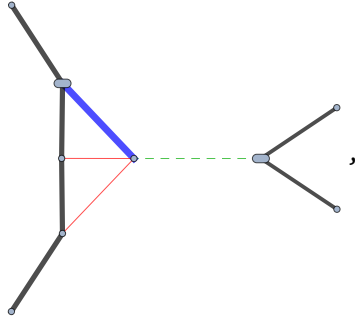

$$G^3 m_1^2 \left( \frac{1}{r^5 \epsilon_d} \left( -2 \hat{n} \cdot \vec{S}_1 \hat{n} \cdot \vec{S}_2 (\hat{n} \cdot \vec{v}_1)^2 + \frac{2}{7} \vec{S}_1 \cdot \vec{S}_2 (\hat{n} \cdot \vec{v}_1)^2 + \frac{4}{7} \hat{n} \cdot \vec{S}_2 \hat{n} \cdot \vec{v}_1 \vec{S}_1 \cdot \vec{v}_1 + \right. \right. \\ \left. \frac{4}{7} \hat{n} \cdot \vec{S}_1 \hat{n} \cdot \vec{v}_1 \vec{S}_2 \cdot \vec{v}_1 + \frac{2}{7} \vec{v}_1 \cdot \vec{v}_1 \hat{n} \cdot \vec{S}_1 \hat{n} \cdot \vec{S}_2 - \frac{4}{35} \vec{S}_1 \cdot \vec{v}_1 \vec{S}_2 \cdot \vec{v}_1 - \frac{2}{35} \vec{S}_1 \cdot \vec{S}_2 \vec{v}_1 \cdot \vec{v}_1 \right) + \\ \frac{1}{r^5} \log \left( \frac{r}{R_0} \right) \left( 6 \hat{n} \cdot \vec{S}_1 \hat{n} \cdot \vec{S}_2 (\hat{n} \cdot \vec{v}_1)^2 - \frac{6}{7} \vec{S}_1 \cdot \vec{S}_2 (\hat{n} \cdot \vec{v}_1)^2 - \frac{12}{7} \hat{n} \cdot \vec{S}_2 \hat{n} \cdot \vec{v}_1 \vec{S}_1 \cdot \vec{v}_1 - \right. \\ \left. \frac{12}{7} \hat{n} \cdot \vec{S}_1 \hat{n} \cdot \vec{v}_1 \vec{S}_2 \cdot \vec{v}_1 - \frac{6}{7} \vec{v}_1 \cdot \vec{v}_1 \hat{n} \cdot \vec{S}_1 \hat{n} \cdot \vec{S}_2 + \frac{12}{35} \vec{S}_1 \cdot \vec{v}_1 \vec{S}_2 \cdot \vec{v}_1 + \frac{6}{35} \vec{S}_1 \cdot \vec{S}_2 \vec{v}_1 \cdot \vec{v}_1 \right) + \frac{1}{r^5} \\ \left( -7 \hat{n} \cdot \vec{S}_1 \hat{n} \cdot \vec{S}_2 (\hat{n} \cdot \vec{v}_1)^2 + \frac{113}{49} \vec{S}_1 \cdot \vec{S}_2 (\hat{n} \cdot \vec{v}_1)^2 + \frac{86}{49} \hat{n} \cdot \vec{S}_2 \hat{n} \cdot \vec{v}_1 \vec{S}_1 \cdot \vec{v}_1 + \frac{58}{49} \hat{n} \cdot \vec{S}_1 \hat{n} \cdot \vec{v}_1 \vec{S}_2 \cdot \vec{v}_1 + \right. \\ \left. \frac{29}{49} \vec{v}_1 \cdot \vec{v}_1 \hat{n} \cdot \vec{S}_1 \hat{n} \cdot \vec{S}_2 - \frac{206 \vec{S}_1 \cdot \vec{v}_1 \vec{S}_2 \cdot \vec{v}_1}{1225} - \frac{313 \vec{S}_1 \cdot \vec{S}_2 \vec{v}_1 \cdot \vec{v}_1}{1225} \right) \Bigg\}$$

{DiagS1S2 [3, 5, 8],

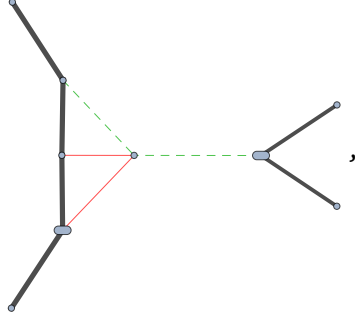

$$\frac{G^3 m_1^2 \left( -96 \hat{n} \times \vec{S}_1 \cdot \vec{v}_1 \hat{n} \times \vec{S}_2 \cdot \vec{v}_1 - 32 \vec{S}_1 \cdot \vec{S}_2 (\hat{n} \cdot \vec{v}_1)^2 + 32 \hat{n} \cdot \vec{S}_1 \hat{n} \cdot \vec{v}_1 \vec{S}_2 \cdot \vec{v}_1 - \frac{128}{5} \vec{S}_1 \cdot \vec{v}_1 \vec{S}_2 \cdot \vec{v}_1 + \frac{128}{5} \vec{S}_1 \cdot \vec{S}_2 \vec{v}_1 \cdot \vec{v}_1 \right)}{r^5} \}$$

{DiagS1S2 [3, 5, 9],

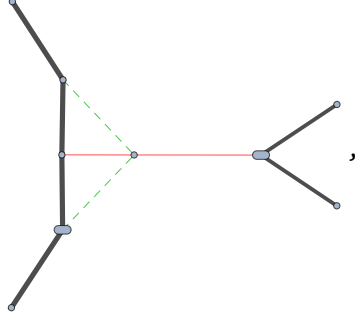

$$\frac{G^3 m_1^2 \left( 32 \hat{n} \times \vec{S}_1 \cdot \vec{v}_1 \hat{n} \times \vec{S}_2 \cdot \vec{v}_2 + \frac{32}{5} \vec{S}_1 \cdot \vec{v}_2 \vec{S}_2 \cdot \vec{v}_1 - \frac{32}{5} \vec{S}_1 \cdot \vec{S}_2 \vec{v}_1 \cdot \vec{v}_2 \right)}{r^5} \}$$

{DiagS1S2 [3, 5, 10],

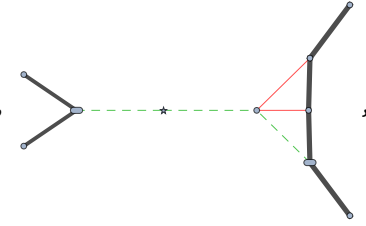

$$\begin{aligned} G^3 m_1^2 & \left( \frac{\frac{68}{75} \vec{S}_1 \cdot \vec{S}_2 - \frac{28}{25} \hat{n} \cdot \vec{S}_1 \hat{n} \cdot \vec{S}_2}{r^3} + \frac{1}{r^4} \left( 8 \hat{n} \cdot \vec{S}_2 \hat{n} \cdot \vec{S}_1 \hat{n} \cdot \vec{v}_1 - \frac{88}{25} \vec{S}_1 \cdot \vec{S}_2 \hat{n} \cdot \vec{v}_1 - 8 \hat{n} \cdot \vec{S}_1 \hat{n} \cdot \vec{S}_2 \hat{n} \cdot \vec{v}_2 + \right. \right. \\ & \left. \frac{88}{25} \hat{n} \cdot \vec{v}_2 \vec{S}_1 \cdot \vec{S}_2 + \frac{28}{25} \hat{n} \cdot \vec{S}_2 \vec{S}_1 \cdot \vec{v}_2 - \frac{28}{25} \hat{n} \cdot \vec{S}_1 \vec{S}_2 \cdot \vec{v}_1 - \frac{28}{25} \hat{n} \cdot \vec{S}_2 \vec{S}_1 \cdot \vec{v}_1 + \frac{28}{25} \hat{n} \cdot \vec{S}_1 \vec{S}_2 \cdot \vec{v}_2 \right) + \frac{1}{r^5} \\ & \left( 68 \hat{n} \cdot \vec{S}_1 \hat{n} \cdot \vec{S}_2 \hat{n} \cdot \vec{v}_1 \hat{n} \cdot \vec{v}_2 - 20 \hat{n} \cdot \vec{v}_1 \vec{S}_1 \cdot \vec{S}_2 \hat{n} \cdot \vec{v}_2 - 8 \hat{n} \cdot \vec{S}_2 \vec{S}_1 \cdot \vec{v}_1 \hat{n} \cdot \vec{v}_2 - 8 \hat{n} \cdot \vec{S}_1 \vec{S}_2 \cdot \vec{v}_1 \hat{n} \cdot \vec{v}_2 - 8 \hat{n} \cdot \vec{S}_2 \hat{n} \cdot \vec{v}_1 \right. \\ & \left. \vec{S}_1 \cdot \vec{v}_2 + \frac{28}{25} \vec{S}_1 \cdot \vec{v}_2 \vec{S}_2 \cdot \vec{v}_1 - 8 \hat{n} \cdot \vec{S}_1 \hat{n} \cdot \vec{v}_1 \vec{S}_2 \cdot \vec{v}_2 + \frac{28}{25} \vec{S}_1 \cdot \vec{v}_1 \vec{S}_2 \cdot \vec{v}_2 - 8 \hat{n} \cdot \vec{S}_1 \hat{n} \cdot \vec{S}_2 \vec{v}_1 \cdot \vec{v}_2 + \frac{88}{25} \vec{S}_1 \cdot \vec{S}_2 \vec{v}_1 \cdot \vec{v}_2 \right) + \\ & \left( \frac{\frac{12}{5} \hat{n} \cdot \vec{S}_1 \hat{n} \cdot \vec{S}_2 - \frac{4}{5} \vec{S}_1 \cdot \vec{S}_2}{r^3} + \frac{1}{r^4} \left( -12 \hat{n} \cdot \vec{S}_2 \hat{n} \cdot \vec{S}_1 \hat{n} \cdot \vec{v}_1 + \frac{12}{5} \vec{S}_1 \cdot \vec{S}_2 \hat{n} \cdot \vec{v}_1 + 12 \hat{n} \cdot \vec{S}_1 \hat{n} \cdot \vec{S}_2 \hat{n} \cdot \vec{v}_2 - \frac{12}{5} \hat{n} \cdot \vec{v}_2 \vec{S}_1 \cdot \vec{S}_2 - \right. \right. \\ & \left. \frac{12}{5} \hat{n} \cdot \vec{S}_2 \vec{S}_1 \cdot \vec{v}_2 + \frac{12}{5} \hat{n} \cdot \vec{S}_1 \vec{S}_2 \cdot \vec{v}_1 + \frac{12}{5} \hat{n} \cdot \vec{S}_2 \vec{S}_1 \cdot \vec{v}_1 - \frac{12}{5} \hat{n} \cdot \vec{S}_1 \vec{S}_2 \cdot \vec{v}_2 \right) + \frac{1}{r^5} \left( -84 \hat{n} \cdot \vec{S}_1 \hat{n} \cdot \vec{S}_2 \hat{n} \cdot \vec{v}_1 \hat{n} \cdot \vec{v}_2 + \right. \\ & \left. 12 \hat{n} \cdot \vec{v}_1 \vec{S}_1 \cdot \vec{S}_2 \hat{n} \cdot \vec{v}_2 + 12 \hat{n} \cdot \vec{S}_2 \vec{S}_1 \cdot \vec{v}_1 \hat{n} \cdot \vec{v}_2 + 12 \hat{n} \cdot \vec{S}_1 \vec{S}_2 \cdot \vec{v}_1 \hat{n} \cdot \vec{v}_2 + 12 \hat{n} \cdot \vec{S}_2 \hat{n} \cdot \vec{v}_1 \vec{S}_1 \cdot \vec{v}_2 - \frac{12}{5} \vec{S}_1 \cdot \vec{v}_2 \right. \end{aligned}$$

$$\begin{aligned}
& \left. \left( \vec{S}_2 \cdot \vec{v}_1 + 12 \hat{n} \cdot \vec{S}_1 \hat{n} \cdot \vec{v}_1 \vec{S}_2 \cdot \vec{v}_2 - \frac{12}{5} \vec{S}_1 \cdot \vec{v}_1 \vec{S}_2 \cdot \vec{v}_2 + 12 \hat{n} \cdot \vec{S}_1 \hat{n} \cdot \vec{S}_2 \vec{v}_1 \cdot \vec{v}_2 - \frac{12}{5} \vec{S}_1 \cdot \vec{S}_2 \vec{v}_1 \cdot \vec{v}_2 \right) \log \left( \frac{r}{R_\theta} \right) + \right. \\
& \frac{1}{\epsilon_d} \left( \frac{\frac{4}{15} \vec{S}_1 \cdot \vec{S}_2 - \frac{4}{5} \hat{n} \cdot \vec{S}_1 \hat{n} \cdot \vec{S}_2}{r^3} + \frac{1}{r^4} \left( 4 \hat{n} \cdot \vec{S}_2 \hat{n} \cdot \vec{S}_1 \hat{n} \cdot \vec{v}_1 - \frac{4}{5} \vec{S}_1 \cdot \vec{S}_2 \hat{n} \cdot \vec{v}_1 - 4 \hat{n} \cdot \vec{S}_1 \hat{n} \cdot \vec{S}_2 \hat{n} \cdot \vec{v}_2 + \right. \right. \\
& \left. \left. \frac{4}{5} \hat{n} \cdot \vec{v}_2 \vec{S}_1 \cdot \vec{S}_2 + \frac{4}{5} \hat{n} \cdot \vec{S}_2 \vec{S}_1 \cdot \vec{v}_2 - \frac{4}{5} \hat{n} \cdot \vec{S}_1 \vec{S}_2 \cdot \vec{v}_1 - \frac{4}{5} \hat{n} \cdot \vec{S}_2 \vec{S}_1 \cdot \vec{v}_1 + \frac{4}{5} \hat{n} \cdot \vec{S}_1 \vec{S}_2 \cdot \vec{v}_2 \right) + \frac{1}{r^5} \right. \\
& \left. \left( 28 \hat{n} \cdot \vec{S}_1 \hat{n} \cdot \vec{S}_2 \hat{n} \cdot \vec{v}_1 \hat{n} \cdot \vec{v}_2 - 4 \hat{n} \cdot \vec{v}_1 \vec{S}_1 \cdot \vec{S}_2 \hat{n} \cdot \vec{v}_2 - 4 \hat{n} \cdot \vec{S}_2 \vec{S}_1 \cdot \vec{v}_1 \hat{n} \cdot \vec{v}_2 - 4 \hat{n} \cdot \vec{S}_1 \vec{S}_2 \cdot \vec{v}_1 \hat{n} \cdot \vec{v}_2 - 4 \hat{n} \cdot \vec{S}_2 \hat{n} \cdot \vec{v}_1 \right. \right. \\
& \left. \left. \vec{S}_1 \cdot \vec{v}_2 + \frac{4}{5} \vec{S}_1 \cdot \vec{v}_2 \vec{S}_2 \cdot \vec{v}_1 - 4 \hat{n} \cdot \vec{S}_1 \hat{n} \cdot \vec{v}_1 \vec{S}_2 \cdot \vec{v}_2 + \frac{4}{5} \vec{S}_1 \cdot \vec{v}_1 \vec{S}_2 \cdot \vec{v}_2 - 4 \hat{n} \cdot \vec{S}_1 \hat{n} \cdot \vec{S}_2 \vec{v}_1 \cdot \vec{v}_2 + \frac{4}{5} \vec{S}_1 \cdot \vec{S}_2 \vec{v}_1 \cdot \vec{v}_2 \right) \right) \Bigg\}
\end{aligned}$$

{DiagS1S2 [3, 5, 11],

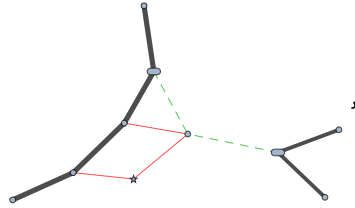

$$\begin{aligned}
& G^3 m_1^2 \left( \frac{1}{r^4} \left( -8 \hat{n} \cdot \vec{S}_2 \hat{n} \cdot \vec{S}_1 \hat{n} \cdot \vec{v}_1 - 8 \hat{n} \cdot \vec{S}_1 \hat{n} \cdot \vec{S}_2 \hat{n} \cdot \vec{v}_1 + \frac{112}{25} \vec{S}_1 \cdot \vec{S}_2 \hat{n} \cdot \vec{v}_1 + \right. \right. \\
& \left. \left. \frac{112}{25} \vec{S}_1 \cdot \vec{S}_2 \hat{n} \cdot \vec{v}_1 + \frac{52}{25} \hat{n} \cdot \vec{S}_2 \vec{S}_1 \cdot \vec{v}_1 - \frac{68}{25} \hat{n} \cdot \vec{S}_1 \vec{S}_2 \cdot \vec{v}_1 + \frac{52}{25} \hat{n} \cdot \vec{S}_2 \vec{S}_1 \cdot \vec{v}_1 - \frac{68}{25} \hat{n} \cdot \vec{S}_1 \vec{S}_2 \cdot \vec{v}_1 \right) + \frac{1}{r^5} \right. \\
& \left( 44 \hat{n} \cdot \vec{S}_1 \hat{n} \cdot \vec{S}_2 (\hat{n} \cdot \vec{v}_1)^2 - \frac{620}{49} \vec{S}_1 \cdot \vec{S}_2 (\hat{n} \cdot \vec{v}_1)^2 - 44 \hat{n} \cdot \vec{S}_1 \hat{n} \cdot \vec{S}_2 \hat{n} \cdot \vec{v}_2 \hat{n} \cdot \vec{v}_1 + 20 \hat{n} \cdot \vec{v}_2 \vec{S}_1 \cdot \vec{S}_2 \hat{n} \cdot \vec{v}_1 - \right. \\
& \left. \frac{736}{49} \hat{n} \cdot \vec{S}_2 \vec{S}_1 \cdot \vec{v}_1 \hat{n} \cdot \vec{v}_1 + 8 \hat{n} \cdot \vec{S}_2 \vec{S}_1 \cdot \vec{v}_2 \hat{n} \cdot \vec{v}_1 - \frac{64}{49} \hat{n} \cdot \vec{S}_1 \vec{S}_2 \cdot \vec{v}_1 \hat{n} \cdot \vec{v}_1 + 8 \hat{n} \cdot \vec{S}_1 \vec{S}_2 \cdot \vec{v}_2 \hat{n} \cdot \vec{v}_1 + \right. \\
& \left. \frac{24}{7} \hat{n} \times \vec{S}_1 \cdot \vec{v}_1 \hat{n} \times \vec{S}_2 \cdot \vec{v}_1 + 8 \hat{n} \cdot \vec{S}_2 \hat{n} \cdot \vec{v}_2 \vec{S}_1 \cdot \vec{v}_1 - 16 \hat{n} \cdot \vec{S}_1 \hat{n} \cdot \vec{v}_2 \vec{S}_2 \cdot \vec{v}_1 + \frac{80}{49} \vec{S}_1 \cdot \vec{v}_1 \vec{S}_2 \cdot \vec{v}_1 + \frac{68}{25} \vec{S}_1 \cdot \vec{v}_2 \vec{S}_2 \cdot \vec{v}_1 - \right. \\
& \left. \frac{52}{25} \vec{S}_1 \cdot \vec{v}_1 \vec{S}_2 \cdot \vec{v}_2 + \frac{80}{49} \hat{n} \cdot \vec{S}_1 \hat{n} \cdot \vec{S}_2 \vec{v}_1 \cdot \vec{v}_1 - \frac{808}{245} \vec{S}_1 \cdot \vec{S}_2 \vec{v}_1 \cdot \vec{v}_1 + 8 \hat{n} \cdot \vec{S}_1 \hat{n} \cdot \vec{S}_2 \vec{v}_1 \cdot \vec{v}_2 - \frac{112}{25} \vec{S}_1 \cdot \vec{S}_2 \vec{v}_1 \cdot \vec{v}_2 \right) + \\
& \left( \frac{1}{r^4} \left( -12 \hat{n} \cdot \vec{S}_2 \hat{n} \cdot \vec{S}_1 \hat{n} \cdot \vec{v}_1 - 12 \hat{n} \cdot \vec{S}_1 \hat{n} \cdot \vec{S}_2 \hat{n} \cdot \vec{v}_1 + \frac{12}{5} \vec{S}_1 \cdot \vec{S}_2 \hat{n} \cdot \vec{v}_1 + \frac{12}{5} \vec{S}_1 \cdot \vec{S}_2 \hat{n} \cdot \vec{v}_1 + \right. \right. \\
& \left. \left. \frac{12}{5} \hat{n} \cdot \vec{S}_2 \vec{S}_1 \cdot \vec{v}_1 + \frac{12}{5} \hat{n} \cdot \vec{S}_1 \vec{S}_2 \cdot \vec{v}_1 + \frac{12}{5} \hat{n} \cdot \vec{S}_2 \vec{S}_1 \cdot \vec{v}_1 + \frac{12}{5} \hat{n} \cdot \vec{S}_1 \vec{S}_2 \cdot \vec{v}_1 \right) + \frac{1}{r^5} \right. \\
& \left( 60 \hat{n} \cdot \vec{S}_1 \hat{n} \cdot \vec{S}_2 (\hat{n} \cdot \vec{v}_1)^2 - \frac{60}{7} \vec{S}_1 \cdot \vec{S}_2 (\hat{n} \cdot \vec{v}_1)^2 - 84 \hat{n} \cdot \vec{S}_1 \hat{n} \cdot \vec{S}_2 \hat{n} \cdot \vec{v}_2 \hat{n} \cdot \vec{v}_1 + 12 \hat{n} \cdot \vec{v}_2 \vec{S}_1 \cdot \vec{S}_2 \hat{n} \cdot \vec{v}_1 - \right. \\
& \left. \frac{120}{7} \hat{n} \cdot \vec{S}_2 \vec{S}_1 \cdot \vec{v}_1 \hat{n} \cdot \vec{v}_1 + 12 \hat{n} \cdot \vec{S}_2 \vec{S}_1 \cdot \vec{v}_2 \hat{n} \cdot \vec{v}_1 - \frac{120}{7} \hat{n} \cdot \vec{S}_1 \vec{S}_2 \cdot \vec{v}_1 \hat{n} \cdot \vec{v}_1 + 12 \hat{n} \cdot \vec{S}_1 \vec{S}_2 \cdot \vec{v}_2 \hat{n} \cdot \vec{v}_1 + \right. \\
& \left. 12 \hat{n} \cdot \vec{S}_2 \hat{n} \cdot \vec{v}_2 \vec{S}_1 \cdot \vec{v}_1 + 12 \hat{n} \cdot \vec{S}_1 \hat{n} \cdot \vec{v}_2 \vec{S}_2 \cdot \vec{v}_1 + \frac{24}{7} \vec{S}_1 \cdot \vec{v}_1 \vec{S}_2 \cdot \vec{v}_1 - \frac{12}{5} \vec{S}_1 \cdot \vec{v}_2 \vec{S}_2 \cdot \vec{v}_1 - \frac{12}{5} \vec{S}_1 \cdot \vec{v}_1 \vec{S}_2 \cdot \vec{v}_2 - \right. \\
& \left. \frac{60}{7} \hat{n} \cdot \vec{S}_1 \hat{n} \cdot \vec{S}_2 \vec{v}_1 \cdot \vec{v}_1 + \frac{12}{7} \vec{S}_1 \cdot \vec{S}_2 \vec{v}_1 \cdot \vec{v}_1 + 12 \hat{n} \cdot \vec{S}_1 \hat{n} \cdot \vec{S}_2 \vec{v}_1 \cdot \vec{v}_2 - \frac{12}{5} \vec{S}_1 \cdot \vec{S}_2 \vec{v}_1 \cdot \vec{v}_2 \right) \log \left( \frac{r}{R_\theta} \right) + \\
& \frac{1}{\epsilon_d} \left( \frac{1}{r^4} \left( 4 \hat{n} \cdot \vec{S}_2 \hat{n} \cdot \vec{S}_1 \hat{n} \cdot \vec{v}_1 + 4 \hat{n} \cdot \vec{S}_1 \hat{n} \cdot \vec{S}_2 \hat{n} \cdot \vec{v}_1 - \frac{4}{5} \vec{S}_1 \cdot \vec{S}_2 \hat{n} \cdot \vec{v}_1 - \frac{4}{5} \vec{S}_1 \cdot \vec{S}_2 \hat{n} \cdot \vec{v}_1 - \right. \right. \\
& \left. \left. \frac{4}{5} \hat{n} \cdot \vec{S}_2 \vec{S}_1 \cdot \vec{v}_1 - \frac{4}{5} \hat{n} \cdot \vec{S}_1 \vec{S}_2 \cdot \vec{v}_1 - \frac{4}{5} \hat{n} \cdot \vec{S}_2 \vec{S}_1 \cdot \vec{v}_1 - \frac{4}{5} \hat{n} \cdot \vec{S}_1 \vec{S}_2 \cdot \vec{v}_1 \right) + \frac{1}{r^5} \right. \\
& \left. \left( -20 \hat{n} \cdot \vec{S}_1 \hat{n} \cdot \vec{S}_2 (\hat{n} \cdot \vec{v}_1)^2 + \frac{20}{7} \vec{S}_1 \cdot \vec{S}_2 (\hat{n} \cdot \vec{v}_1)^2 + 28 \hat{n} \cdot \vec{S}_1 \hat{n} \cdot \vec{S}_2 \hat{n} \cdot \vec{v}_2 \hat{n} \cdot \vec{v}_1 - 4 \hat{n} \cdot \vec{v}_2 \vec{S}_1 \cdot \vec{S}_2 \hat{n} \cdot \vec{v}_1 + \right. \right.
\end{aligned}$$

$$\begin{aligned} & \frac{40}{7} \hat{n} \cdot \vec{S}_2 \vec{S}_1 \cdot \vec{v}_1 \hat{n} \cdot \vec{v}_1 - 4 \hat{n} \cdot \vec{S}_2 \vec{S}_1 \cdot \vec{v}_2 \hat{n} \cdot \vec{v}_1 + \frac{40}{7} \hat{n} \cdot \vec{S}_1 \vec{S}_2 \cdot \vec{v}_1 \hat{n} \cdot \vec{v}_1 - 4 \hat{n} \cdot \vec{S}_1 \vec{S}_2 \cdot \vec{v}_2 \hat{n} \cdot \vec{v}_1 - \\ & 4 \hat{n} \cdot \vec{S}_2 \hat{n} \cdot \vec{v}_2 \vec{S}_1 \cdot \vec{v}_1 - 4 \hat{n} \cdot \vec{S}_1 \hat{n} \cdot \vec{v}_2 \vec{S}_2 \cdot \vec{v}_1 - \frac{8}{7} \vec{S}_1 \cdot \vec{v}_1 \vec{S}_2 \cdot \vec{v}_1 + \frac{4}{5} \vec{S}_1 \cdot \vec{v}_2 \vec{S}_2 \cdot \vec{v}_1 + \frac{4}{5} \vec{S}_1 \cdot \vec{v}_1 \vec{S}_2 \cdot \vec{v}_2 + \\ & \frac{20}{7} \hat{n} \cdot \vec{S}_1 \hat{n} \cdot \vec{S}_2 \vec{v}_1 \cdot \vec{v}_1 - \frac{4}{7} \vec{S}_1 \cdot \vec{S}_2 \vec{v}_1 \cdot \vec{v}_1 - 4 \hat{n} \cdot \vec{S}_1 \hat{n} \cdot \vec{S}_2 \vec{v}_1 \cdot \vec{v}_2 + \frac{4}{5} \vec{S}_1 \cdot \vec{S}_2 \vec{v}_1 \cdot \vec{v}_2 \Big) \Big) \Big) \Big) \Big) \Big\} \end{aligned}$$

{DiagS1S2[3, 5, 12],

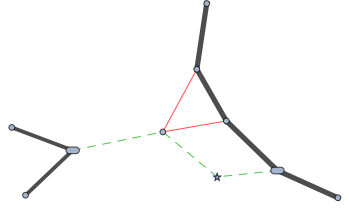

,

$$\begin{aligned} G^3 m_1^2 & \left( \frac{\frac{20}{3} \vec{S}_1 \cdot \vec{S}_2 - 4 \hat{n} \cdot \vec{S}_1 \hat{n} \cdot \vec{S}_2}{r^3} + \frac{1}{r^4} \left( 12 \hat{n} \cdot \vec{S}_2 \hat{n} \cdot \vec{S}_1 \hat{n} \cdot \vec{v}_1 + 32 \hat{n} \cdot \vec{S}_1 \hat{n} \cdot \vec{S}_2 \hat{n} \cdot \vec{v}_1 - \right. \right. \\ & \frac{456}{25} \vec{S}_1 \cdot \vec{S}_2 \hat{n} \cdot \vec{v}_1 - \frac{244}{25} \vec{S}_1 \cdot \vec{S}_2 \hat{n} \cdot \vec{v}_1 - 44 \hat{n} \cdot \vec{S}_1 \hat{n} \cdot \vec{S}_2 \hat{n} \cdot \vec{v}_2 + 28 \hat{n} \cdot \vec{v}_2 \vec{S}_1 \cdot \vec{S}_2 - \frac{76}{25} \hat{n} \cdot \vec{S}_2 \vec{S}_1 \cdot \vec{v}_1 + \\ & 4 \hat{n} \cdot \vec{S}_2 \vec{S}_1 \cdot \vec{v}_2 + \frac{16}{25} \hat{n} \cdot \vec{S}_1 \vec{S}_2 \cdot \vec{v}_1 - \frac{24}{25} \hat{n} \cdot \vec{S}_2 \vec{S}_1 \cdot \vec{v}_1 - \frac{116}{25} \hat{n} \cdot \vec{S}_1 \vec{S}_2 \cdot \vec{v}_1 + 4 \hat{n} \cdot \vec{S}_1 \vec{S}_2 \cdot \vec{v}_2 \Big) + \frac{1}{r^5} \\ & \left( -68 \hat{n} \cdot \vec{S}_1 \hat{n} \cdot \vec{S}_2 (\hat{n} \cdot \vec{v}_1)^2 + \frac{1404}{49} \vec{S}_1 \cdot \vec{S}_2 (\hat{n} \cdot \vec{v}_1)^2 + 120 \hat{n} \cdot \vec{S}_1 \hat{n} \cdot \vec{S}_2 \hat{n} \cdot \vec{v}_2 \hat{n} \cdot \vec{v}_1 - 56 \hat{n} \cdot \vec{v}_2 \vec{S}_1 \cdot \vec{S}_2 \hat{n} \cdot \vec{v}_1 + \right. \\ & \frac{736}{49} \hat{n} \cdot \vec{S}_2 \vec{S}_1 \cdot \vec{v}_1 \hat{n} \cdot \vec{v}_1 - 12 \hat{n} \cdot \vec{S}_2 \vec{S}_1 \cdot \vec{v}_2 \hat{n} \cdot \vec{v}_1 + \frac{456}{49} \hat{n} \cdot \vec{S}_1 \vec{S}_2 \cdot \vec{v}_1 \hat{n} \cdot \vec{v}_1 - 12 \hat{n} \cdot \vec{S}_1 \vec{S}_2 \cdot \vec{v}_2 \hat{n} \cdot \vec{v}_1 + \\ & \frac{32}{7} \hat{n} \times \vec{S}_1 \cdot \vec{v}_1 \hat{n} \times \vec{S}_2 \cdot \vec{v}_1 - 12 \hat{n} \cdot \vec{S}_2 \hat{n} \cdot \vec{v}_2 \vec{S}_1 \cdot \vec{v}_1 - 4 \hat{n} \cdot \vec{S}_1 \hat{n} \cdot \vec{v}_2 \vec{S}_2 \cdot \vec{v}_1 + \frac{352 \vec{S}_1 \cdot \vec{v}_1 \vec{S}_2 \cdot \vec{v}_1}{1225} - \frac{16}{25} \vec{S}_1 \cdot \vec{v}_2 \vec{S}_2 \cdot \vec{v}_1 + \\ & \frac{24}{25} \vec{S}_1 \cdot \vec{v}_1 \vec{S}_2 \cdot \vec{v}_2 + \frac{312}{49} \hat{n} \cdot \vec{S}_1 \hat{n} \cdot \vec{S}_2 \vec{v}_1 \cdot \vec{v}_1 - \frac{6544 \vec{S}_1 \cdot \vec{S}_2 \vec{v}_1 \cdot \vec{v}_1}{1225} - 12 \hat{n} \cdot \vec{S}_1 \hat{n} \cdot \vec{S}_2 \vec{v}_1 \cdot \vec{v}_2 + \frac{244}{25} \vec{S}_1 \cdot \vec{S}_2 \vec{v}_1 \cdot \vec{v}_2 \Big) + \\ & \left( \frac{24 \hat{n} \cdot \vec{S}_1 \hat{n} \cdot \vec{S}_2 - 8 \vec{S}_1 \cdot \vec{S}_2}{r^3} + \frac{1}{r^4} \left( -36 \hat{n} \cdot \vec{S}_2 \hat{n} \cdot \vec{S}_1 \hat{n} \cdot \vec{v}_1 - 84 \hat{n} \cdot \vec{S}_1 \hat{n} \cdot \vec{S}_2 \hat{n} \cdot \vec{v}_1 + \frac{84}{5} \vec{S}_1 \cdot \vec{S}_2 \hat{n} \cdot \vec{v}_1 + \right. \right. \\ & \frac{36}{5} \vec{S}_1 \cdot \vec{S}_2 \hat{n} \cdot \vec{v}_1 + 120 \hat{n} \cdot \vec{S}_1 \hat{n} \cdot \vec{S}_2 \hat{n} \cdot \vec{v}_2 - 24 \hat{n} \cdot \vec{v}_2 \vec{S}_1 \cdot \vec{S}_2 + \frac{84}{5} \hat{n} \cdot \vec{S}_2 \vec{S}_1 \cdot \vec{v}_1 - \\ & 24 \hat{n} \cdot \vec{S}_2 \vec{S}_1 \cdot \vec{v}_2 + \frac{36}{5} \hat{n} \cdot \vec{S}_1 \vec{S}_2 \cdot \vec{v}_1 + \frac{36}{5} \hat{n} \cdot \vec{S}_2 \vec{S}_1 \cdot \vec{v}_1 + \frac{84}{5} \hat{n} \cdot \vec{S}_1 \vec{S}_2 \cdot \vec{v}_1 - 24 \hat{n} \cdot \vec{S}_1 \vec{S}_2 \cdot \vec{v}_2 \Big) + \frac{1}{r^5} \\ & \left( 108 \hat{n} \cdot \vec{S}_1 \hat{n} \cdot \vec{S}_2 (\hat{n} \cdot \vec{v}_1)^2 - \frac{108}{7} \vec{S}_1 \cdot \vec{S}_2 (\hat{n} \cdot \vec{v}_1)^2 - 252 \hat{n} \cdot \vec{S}_1 \hat{n} \cdot \vec{S}_2 \hat{n} \cdot \vec{v}_2 \hat{n} \cdot \vec{v}_1 + 36 \hat{n} \cdot \vec{v}_2 \vec{S}_1 \cdot \vec{S}_2 \hat{n} \cdot \vec{v}_1 - \right. \\ & \frac{216}{7} \hat{n} \cdot \vec{S}_2 \vec{S}_1 \cdot \vec{v}_1 \hat{n} \cdot \vec{v}_1 + 36 \hat{n} \cdot \vec{S}_2 \vec{S}_1 \cdot \vec{v}_2 \hat{n} \cdot \vec{v}_1 - \frac{216}{7} \hat{n} \cdot \vec{S}_1 \vec{S}_2 \cdot \vec{v}_1 \hat{n} \cdot \vec{v}_1 + 36 \hat{n} \cdot \vec{S}_1 \vec{S}_2 \cdot \vec{v}_2 \hat{n} \cdot \vec{v}_1 + \\ & 36 \hat{n} \cdot \vec{S}_2 \hat{n} \cdot \vec{v}_2 \vec{S}_1 \cdot \vec{v}_1 + 36 \hat{n} \cdot \vec{S}_1 \hat{n} \cdot \vec{v}_2 \vec{S}_2 \cdot \vec{v}_1 + \frac{216}{35} \vec{S}_1 \cdot \vec{v}_1 \vec{S}_2 \cdot \vec{v}_1 - \frac{36}{5} \vec{S}_1 \cdot \vec{v}_2 \vec{S}_2 \cdot \vec{v}_1 - \frac{36}{5} \vec{S}_1 \cdot \vec{v}_1 \vec{S}_2 \cdot \vec{v}_2 - \\ & \frac{108}{7} \hat{n} \cdot \vec{S}_1 \hat{n} \cdot \vec{S}_2 \vec{v}_1 \cdot \vec{v}_1 + \frac{108}{35} \vec{S}_1 \cdot \vec{S}_2 \vec{v}_1 \cdot \vec{v}_1 + 36 \hat{n} \cdot \vec{S}_1 \hat{n} \cdot \vec{S}_2 \vec{v}_1 \cdot \vec{v}_2 - \frac{36}{5} \vec{S}_1 \cdot \vec{S}_2 \vec{v}_1 \cdot \vec{v}_2 \Big) \log \left( \frac{r}{R_\theta} \right) + \\ & \frac{1}{\epsilon_d} \left( \frac{\frac{8}{3} \vec{S}_1 \cdot \vec{S}_2 - 8 \hat{n} \cdot \vec{S}_1 \hat{n} \cdot \vec{S}_2}{r^3} + \frac{1}{r^4} \left( 12 \hat{n} \cdot \vec{S}_2 \hat{n} \cdot \vec{S}_1 \hat{n} \cdot \vec{v}_1 + 28 \hat{n} \cdot \vec{S}_1 \hat{n} \cdot \vec{S}_2 \hat{n} \cdot \vec{v}_1 - \frac{28}{5} \vec{S}_1 \cdot \vec{S}_2 \hat{n} \cdot \vec{v}_1 - \right. \right. \end{aligned}$$

$$\begin{aligned}
& \frac{12}{5} \vec{S}_1 \cdot \vec{S}_2 \hat{n} \cdot \vec{v}_1 - 40 \hat{n} \cdot \vec{S}_1 \hat{n} \cdot \vec{S}_2 \hat{n} \cdot \vec{v}_2 + 8 \hat{n} \cdot \vec{v}_2 \vec{S}_1 \cdot \vec{S}_2 - \frac{28}{5} \hat{n} \cdot \vec{S}_2 \vec{S}_1 \cdot \vec{v}_1 + \\
& 8 \hat{n} \cdot \vec{S}_2 \vec{S}_1 \cdot \vec{v}_2 - \frac{12}{5} \hat{n} \cdot \vec{S}_1 \vec{S}_2 \cdot \vec{v}_1 - \frac{12}{5} \hat{n} \cdot \vec{S}_2 \vec{S}_1 \cdot \vec{v}_1 - \frac{28}{5} \hat{n} \cdot \vec{S}_1 \vec{S}_2 \cdot \vec{v}_1 + 8 \hat{n} \cdot \vec{S}_1 \vec{S}_2 \cdot \vec{v}_2 \Bigg) + \frac{1}{r^5} \\
& \left( -36 \hat{n} \cdot \vec{S}_1 \hat{n} \cdot \vec{S}_2 (\hat{n} \cdot \vec{v}_1)^2 + \frac{36}{7} \vec{S}_1 \cdot \vec{S}_2 (\hat{n} \cdot \vec{v}_1)^2 + 84 \hat{n} \cdot \vec{S}_1 \hat{n} \cdot \vec{S}_2 \hat{n} \cdot \vec{v}_2 \hat{n} \cdot \vec{v}_1 - 12 \hat{n} \cdot \vec{v}_2 \vec{S}_1 \cdot \vec{S}_2 \hat{n} \cdot \vec{v}_1 + \right. \\
& \frac{72}{7} \hat{n} \cdot \vec{S}_2 \vec{S}_1 \cdot \vec{v}_1 \hat{n} \cdot \vec{v}_1 - 12 \hat{n} \cdot \vec{S}_2 \vec{S}_1 \cdot \vec{v}_2 \hat{n} \cdot \vec{v}_1 + \frac{72}{7} \hat{n} \cdot \vec{S}_1 \vec{S}_2 \cdot \vec{v}_1 \hat{n} \cdot \vec{v}_1 - 12 \hat{n} \cdot \vec{S}_1 \vec{S}_2 \cdot \vec{v}_2 \hat{n} \cdot \vec{v}_1 - \\
& 12 \hat{n} \cdot \vec{S}_2 \hat{n} \cdot \vec{v}_2 \vec{S}_1 \cdot \vec{v}_1 - 12 \hat{n} \cdot \vec{S}_1 \hat{n} \cdot \vec{v}_2 \vec{S}_2 \cdot \vec{v}_1 - \frac{72}{35} \vec{S}_1 \cdot \vec{v}_1 \vec{S}_2 \cdot \vec{v}_1 + \frac{12}{5} \vec{S}_1 \cdot \vec{v}_2 \vec{S}_2 \cdot \vec{v}_1 + \frac{12}{5} \vec{S}_1 \cdot \vec{v}_1 \vec{S}_2 \cdot \vec{v}_2 + \\
& \left. \frac{36}{7} \hat{n} \cdot \vec{S}_1 \hat{n} \cdot \vec{S}_2 \vec{v}_1 \cdot \vec{v}_1 - \frac{36}{35} \vec{S}_1 \cdot \vec{S}_2 \vec{v}_1 \cdot \vec{v}_1 - 12 \hat{n} \cdot \vec{S}_1 \hat{n} \cdot \vec{S}_2 \vec{v}_1 \cdot \vec{v}_2 + \frac{12}{5} \vec{S}_1 \cdot \vec{S}_2 \vec{v}_1 \cdot \vec{v}_2 \right) \Bigg] \Bigg\}
\end{aligned}$$

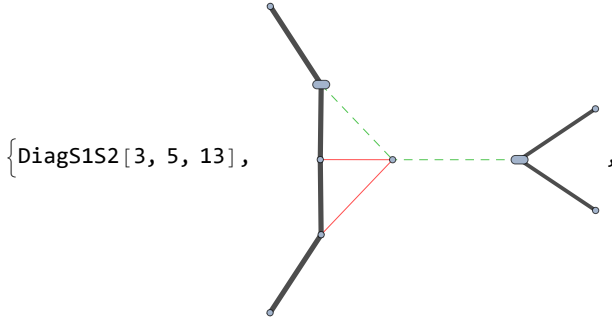

$$\begin{aligned}
& G^3 m_1^2 \left( \frac{1}{r^4} \left( -16 \hat{n} \cdot \vec{v}_1 \vec{S}_1 \cdot \vec{S}_2 + \frac{16}{5} \hat{n} \cdot \vec{v}_2 \vec{S}_1 \cdot \vec{S}_2 - \frac{16}{5} \hat{n} \cdot \vec{S}_2 \vec{S}_1 \cdot \vec{a}_2 - \right. \right. \\
& 16 \hat{n} \cdot \vec{a}_1 \vec{S}_1 \cdot \vec{S}_2 + \frac{16}{5} \hat{n} \cdot \vec{a}_2 \vec{S}_1 \cdot \vec{S}_2 - \frac{16}{5} \hat{n} \cdot \vec{S}_2 \vec{S}_1 \cdot \vec{v}_2 + 16 \hat{n} \cdot \vec{S}_1 \vec{S}_2 \cdot \vec{a}_1 + 16 \hat{n} \cdot \vec{S}_1 \vec{S}_2 \cdot \vec{v}_1 \Bigg) + \frac{1}{r^5} \\
& \left( 7 \hat{n} \cdot \vec{S}_1 \hat{n} \cdot \vec{S}_2 (\hat{n} \cdot \vec{v}_1)^2 + \frac{867}{49} \vec{S}_1 \cdot \vec{S}_2 (\hat{n} \cdot \vec{v}_1)^2 - \frac{86}{49} \hat{n} \cdot \vec{S}_2 \vec{S}_1 \cdot \vec{v}_1 \hat{n} \cdot \vec{v}_1 - \frac{1038}{49} \hat{n} \cdot \vec{S}_1 \vec{S}_2 \cdot \vec{v}_1 \hat{n} \cdot \vec{v}_1 - \right. \\
& 28 \hat{n} \cdot \vec{S}_1 \cdot \vec{v}_1 \hat{n} \cdot \vec{S}_2 \cdot \vec{v}_1 - 12 \hat{n} \cdot \vec{S}_1 \cdot \vec{v}_2 \hat{n} \cdot \vec{S}_2 \cdot \vec{v}_2 + 4 (\hat{n} \cdot \vec{v}_2)^2 \vec{S}_1 \cdot \vec{S}_2 - 4 \hat{n} \cdot \vec{S}_2 \hat{n} \cdot \vec{v}_2 \vec{S}_1 \cdot \vec{v}_2 - \\
& \frac{1754 \vec{S}_1 \cdot \vec{v}_1 \vec{S}_2 \cdot \vec{v}_1}{1225} - \frac{8}{5} \vec{S}_1 \cdot \vec{v}_2 \vec{S}_2 \cdot \vec{v}_2 + \frac{1147}{49} \hat{n} \cdot \vec{S}_1 \hat{n} \cdot \vec{S}_2 \vec{v}_1 \cdot \vec{v}_1 - \frac{15367 \vec{S}_1 \cdot \vec{S}_2 \vec{v}_1 \cdot \vec{v}_1}{1225} + \frac{8}{5} \vec{S}_1 \cdot \vec{S}_2 \vec{v}_2 \cdot \vec{v}_2 \Bigg) + \\
& \frac{1}{r^5} \left( -6 \hat{n} \cdot \vec{S}_1 \hat{n} \cdot \vec{S}_2 (\hat{n} \cdot \vec{v}_1)^2 + \frac{6}{7} \vec{S}_1 \cdot \vec{S}_2 (\hat{n} \cdot \vec{v}_1)^2 + \frac{12}{7} \hat{n} \cdot \vec{S}_2 \vec{S}_1 \cdot \vec{v}_1 \hat{n} \cdot \vec{v}_1 + \frac{12}{7} \hat{n} \cdot \vec{S}_1 \vec{S}_2 \cdot \vec{v}_1 \hat{n} \cdot \vec{v}_1 - \right. \\
& \frac{12}{35} \vec{S}_1 \cdot \vec{v}_1 \vec{S}_2 \cdot \vec{v}_1 + \frac{6}{7} \hat{n} \cdot \vec{S}_1 \hat{n} \cdot \vec{S}_2 \vec{v}_1 \cdot \vec{v}_1 - \frac{6}{35} \vec{S}_1 \cdot \vec{S}_2 \vec{v}_1 \cdot \vec{v}_1 \Bigg) \log \left( \frac{r}{R_\theta} \right) + \frac{1}{r^5 \in_d} \\
& \left( 2 \hat{n} \cdot \vec{S}_1 \hat{n} \cdot \vec{S}_2 (\hat{n} \cdot \vec{v}_1)^2 - \frac{2}{7} \vec{S}_1 \cdot \vec{S}_2 (\hat{n} \cdot \vec{v}_1)^2 - \frac{4}{7} \hat{n} \cdot \vec{S}_2 \vec{S}_1 \cdot \vec{v}_1 \hat{n} \cdot \vec{v}_1 - \frac{4}{7} \hat{n} \cdot \vec{S}_1 \vec{S}_2 \cdot \vec{v}_1 \hat{n} \cdot \vec{v}_1 + \right. \\
& \left. \frac{4}{35} \vec{S}_1 \cdot \vec{v}_1 \vec{S}_2 \cdot \vec{v}_1 - \frac{2}{7} \hat{n} \cdot \vec{S}_1 \hat{n} \cdot \vec{S}_2 \vec{v}_1 \cdot \vec{v}_1 + \frac{2}{35} \vec{S}_1 \cdot \vec{S}_2 \vec{v}_1 \cdot \vec{v}_1 \right) \Bigg\}
\end{aligned}$$

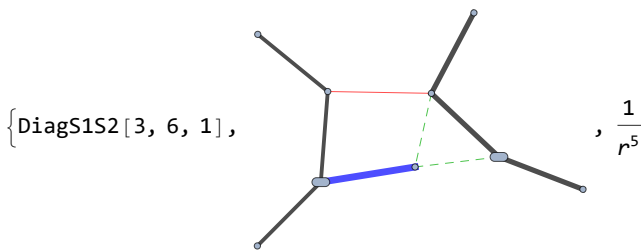

$$G^3 m_1 m_2 \left( 4 \hat{n} \times \vec{S}_1 \cdot \vec{v}_2 \hat{n} \times \vec{S}_2 \cdot \vec{v}_1 - 4 \hat{n} \times \vec{S}_1 \cdot \vec{v}_1 \hat{n} \times \vec{S}_2 \cdot \vec{v}_2 + 4 \vec{S}_1 \cdot \vec{S}_2 \hat{n} \cdot \vec{v}_1 \hat{n} \cdot \vec{v}_2 - 4 \hat{n} \cdot \vec{S}_1 \hat{n} \cdot \vec{v}_2 \vec{S}_2 \cdot \vec{v}_1 - 4 \vec{v}_1 \cdot \vec{v}_2 \hat{n} \cdot \vec{S}_1 \hat{n} \cdot \vec{S}_2 + \vec{S}_1 \cdot \vec{v}_1 \vec{S}_2 \cdot \vec{v}_2 + \vec{S}_1 \cdot \vec{S}_2 \vec{v}_1 \cdot \vec{v}_2 \right) \Big\}$$

$$\left\{ \text{DiagS1S2}[3, 6, 2], \right. , \frac{1}{r^5}$$
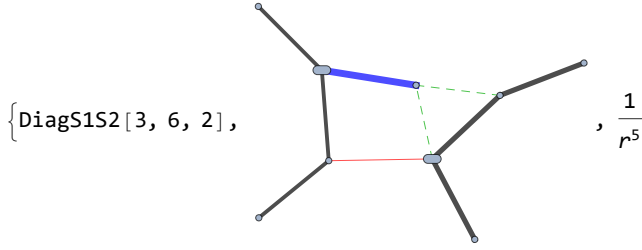

$$G^3 m_1 m_2 \left( 16 \hat{n} \times \vec{S}_1 \cdot \vec{v}_2 \hat{n} \times \vec{S}_2 \cdot \vec{v}_1 - 16 \hat{n} \times \vec{S}_1 \cdot \vec{v}_1 \hat{n} \times \vec{S}_2 \cdot \vec{v}_2 + 16 \vec{S}_1 \cdot \vec{S}_2 \hat{n} \cdot \vec{v}_1 \hat{n} \cdot \vec{v}_2 - 16 \hat{n} \cdot \vec{S}_1 \hat{n} \cdot \vec{v}_2 \vec{S}_2 \cdot \vec{v}_1 - 16 \vec{v}_1 \cdot \vec{v}_2 \hat{n} \cdot \vec{S}_1 \hat{n} \cdot \vec{S}_2 + 4 \vec{S}_1 \cdot \vec{v}_1 \vec{S}_2 \cdot \vec{v}_2 + 4 \vec{S}_1 \cdot \vec{S}_2 \vec{v}_1 \cdot \vec{v}_2 \right) \Big\}$$

$$\left\{ \text{DiagS1S2}[3, 6, 3], \right. , \frac{1}{r^5}$$
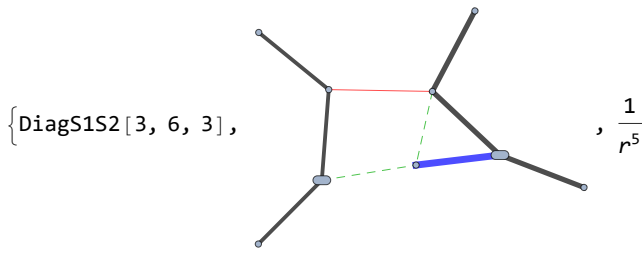

$$G^3 m_1 m_2 \left( 16 \hat{n} \times \vec{S}_1 \cdot \vec{v}_1 \hat{n} \times \vec{S}_2 \cdot \vec{v}_1 + 4 \vec{S}_1 \cdot \vec{S}_2 (\hat{n} \cdot \vec{v}_1)^2 - 4 \hat{n} \cdot \vec{S}_1 \hat{n} \cdot \vec{v}_1 \vec{S}_2 \cdot \vec{v}_1 + 12 \vec{v}_1 \cdot \vec{v}_1 \hat{n} \cdot \vec{S}_1 \hat{n} \cdot \vec{S}_2 + 5 \vec{S}_1 \cdot \vec{v}_1 \vec{S}_2 \cdot \vec{v}_1 - 11 \vec{S}_1 \cdot \vec{S}_2 \vec{v}_1 \cdot \vec{v}_1 \right) \Big\}$$

$$\left\{ \text{DiagS1S2}[3, 6, 4], \right. , \frac{1}{r^5}$$
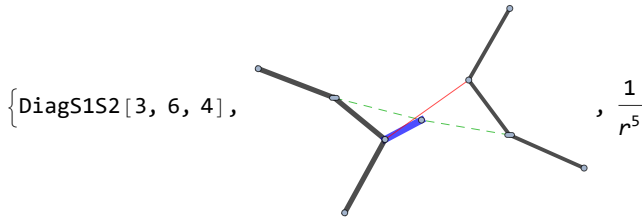

$$G^3 m_1 m_2 \left( 12 \hat{n} \times \vec{S}_1 \cdot \vec{v}_1 \hat{n} \times \vec{S}_2 \cdot \vec{v}_1 + 216 \hat{n} \cdot \vec{S}_1 \hat{n} \cdot \vec{S}_2 (\hat{n} \cdot \vec{v}_1)^2 - 24 \vec{S}_1 \cdot \vec{S}_2 (\hat{n} \cdot \vec{v}_1)^2 - 72 \hat{n} \cdot \vec{S}_2 \hat{n} \cdot \vec{v}_1 \vec{S}_1 \cdot \vec{v}_1 - 48 \hat{n} \cdot \vec{S}_1 \hat{n} \cdot \vec{v}_1 \vec{S}_2 \cdot \vec{v}_1 - 24 \vec{v}_1 \cdot \vec{v}_1 \hat{n} \cdot \vec{S}_1 \hat{n} \cdot \vec{S}_2 + 15 \vec{S}_1 \cdot \vec{v}_1 \vec{S}_2 \cdot \vec{v}_1 - 3 \vec{S}_1 \cdot \vec{S}_2 \vec{v}_1 \cdot \vec{v}_1 \right) \Big\}$$

$$\left\{ \text{DiagS1S2}[3, 6, 5], \right. , \frac{1}{r^5}$$
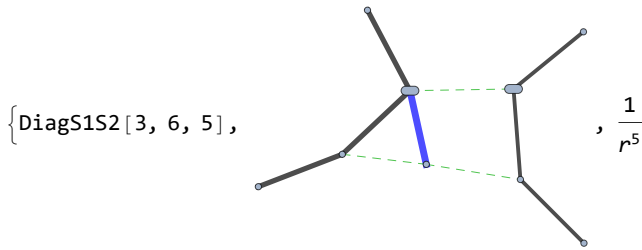

$$G^3 m_1 m_2 \left( 12 \hat{n} \times \vec{S}_1 \cdot \vec{v}_2 \hat{n} \times \vec{S}_2 \cdot \vec{v}_1 + 12 \hat{n} \times \vec{S}_1 \cdot \vec{v}_1 \hat{n} \times \vec{S}_2 \cdot \vec{v}_2 + 24 \vec{S}_1 \cdot \vec{S}_2 \hat{n} \cdot \vec{v}_1 \hat{n} \cdot \vec{v}_2 - 12 \hat{n} \cdot \vec{S}_1 \hat{n} \cdot \vec{v}_2 \vec{S}_2 \cdot \vec{v}_1 - 12 \hat{n} \cdot \vec{S}_1 \hat{n} \cdot \vec{v}_1 \vec{S}_2 \cdot \vec{v}_2 + 16 \vec{v}_1 \cdot \vec{v}_2 \hat{n} \cdot \vec{S}_1 \hat{n} \cdot \vec{S}_2 + 8 \vec{S}_1 \cdot \vec{v}_2 \vec{S}_2 \cdot \vec{v}_1 + 8 \vec{S}_1 \cdot \vec{v}_1 \vec{S}_2 \cdot \vec{v}_2 - 32 \vec{S}_1 \cdot \vec{S}_2 \vec{v}_1 \cdot \vec{v}_2 \right) \Big\}$$

$\{\text{DiagS1S2}[3, 6, 6],$ 
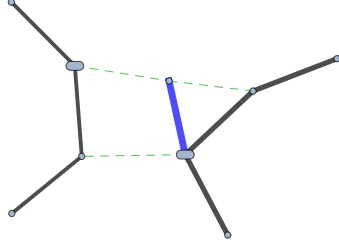
 $, \frac{1}{r^5}$ 

$$G^3 m_1 m_2 \left( -48 \hat{n} \times \vec{S}_1 \cdot \vec{v}_2 \hat{n} \times \vec{S}_2 \cdot \vec{v}_1 + 8 \hat{n} \times \vec{S}_1 \cdot \vec{v}_1 \hat{n} \times \vec{S}_2 \cdot \vec{v}_2 - 24 \vec{S}_1 \cdot \vec{S}_2 \hat{n} \cdot \vec{v}_1 \hat{n} \cdot \vec{v}_2 + \right. \\ \left. 16 \hat{n} \cdot \vec{S}_2 \hat{n} \cdot \vec{v}_2 \vec{S}_1 \cdot \vec{v}_1 + 8 \hat{n} \cdot \vec{S}_1 \hat{n} \cdot \vec{v}_1 \vec{S}_2 \cdot \vec{v}_2 - 8 \vec{v}_1 \cdot \vec{v}_2 \hat{n} \cdot \vec{S}_1 \hat{n} \cdot \vec{S}_2 - 16 \vec{S}_1 \cdot \vec{v}_1 \vec{S}_2 \cdot \vec{v}_2 + 24 \vec{S}_1 \cdot \vec{S}_2 \vec{v}_1 \cdot \vec{v}_2 \right) \}$$

 $\{\text{DiagS1S2}[3, 6, 7],$ 
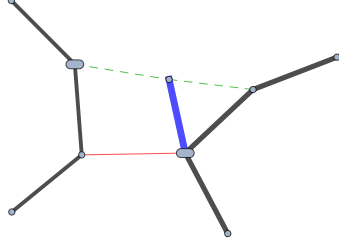
 $, \frac{1}{r^5}$ 

$$G^3 m_1 m_2 \left( 56 \hat{n} \times \vec{S}_1 \cdot \vec{v}_1 \hat{n} \times \vec{S}_2 \cdot \vec{v}_1 - 8 \vec{S}_1 \cdot \vec{S}_2 (\hat{n} \cdot \vec{v}_1)^2 + 16 \hat{n} \cdot \vec{S}_2 \hat{n} \cdot \vec{v}_1 \vec{S}_1 \cdot \vec{v}_1 - \right. \\ \left. 8 \hat{n} \cdot \vec{S}_1 \hat{n} \cdot \vec{v}_1 \vec{S}_2 \cdot \vec{v}_1 - 8 \vec{v}_1 \cdot \vec{v}_1 \hat{n} \cdot \vec{S}_1 \hat{n} \cdot \vec{S}_2 + 16 \vec{S}_1 \cdot \vec{v}_1 \vec{S}_2 \cdot \vec{v}_1 - 8 \vec{S}_1 \cdot \vec{S}_2 \vec{v}_1 \cdot \vec{v}_1 \right) \}$$

 $\{\text{DiagS1S2}[3, 6, 8],$ 
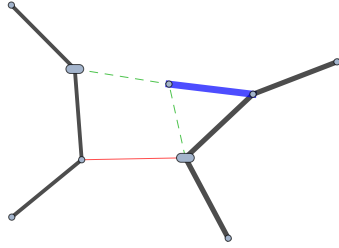
 $, \frac{1}{r^5}$ 

$$G^3 m_1 m_2 \left( -16 \hat{n} \times \vec{S}_1 \cdot \vec{v}_1 \hat{n} \times \vec{S}_2 \cdot \vec{v}_1 - 288 \hat{n} \cdot \vec{S}_1 \hat{n} \cdot \vec{S}_2 (\hat{n} \cdot \vec{v}_1)^2 + 32 \vec{S}_1 \cdot \vec{S}_2 (\hat{n} \cdot \vec{v}_1)^2 + \right. \\ \left. 96 \hat{n} \cdot \vec{S}_2 \hat{n} \cdot \vec{v}_1 \vec{S}_1 \cdot \vec{v}_1 + 64 \hat{n} \cdot \vec{S}_1 \hat{n} \cdot \vec{v}_1 \vec{S}_2 \cdot \vec{v}_1 + 32 \vec{v}_1 \cdot \vec{v}_1 \hat{n} \cdot \vec{S}_1 \hat{n} \cdot \vec{S}_2 - 20 \vec{S}_1 \cdot \vec{v}_1 \vec{S}_2 \cdot \vec{v}_1 + 4 \vec{S}_1 \cdot \vec{S}_2 \vec{v}_1 \cdot \vec{v}_1 \right) \}$$

 $\{\text{DiagS1S2}[3, 6, 9],$ 
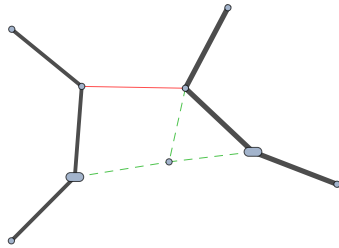
 $,$ 

$$G^3 m_1 m_2 \left( \frac{1}{r^4} \left( \vec{S}_1 \cdot \vec{S}_2 \hat{n} \cdot \vec{a}_1 - \vec{S}_2 \cdot \vec{a}_1 \hat{n} \cdot \vec{S}_1 + 12 \hat{n} \cdot \vec{S}_2 \hat{n} \cdot \vec{S}_1 \hat{n} \cdot \vec{v}_1 - 16 \hat{n} \cdot \vec{S}_1 \hat{n} \cdot \vec{S}_2 \hat{n} \cdot \vec{v}_1 - \right. \right. \\ \left. \left. \vec{S}_1 \cdot \vec{S}_2 \hat{n} \cdot \vec{v}_1 - \vec{S}_1 \cdot \vec{S}_2 \hat{n} \cdot \vec{v}_1 + 4 \hat{n} \cdot \vec{S}_2 \vec{S}_1 \cdot \vec{v}_1 - 2 \hat{n} \cdot \vec{S}_1 \vec{S}_2 \cdot \vec{v}_1 - 3 \hat{n} \cdot \vec{S}_2 \vec{S}_1 \cdot \vec{v}_1 + 5 \hat{n} \cdot \vec{S}_1 \vec{S}_2 \cdot \vec{v}_1 \right) + \frac{1}{r^5} \right. \\ \left. \left( -8 \hat{n} \times \vec{S}_1 \cdot \vec{v}_1 \hat{n} \times \vec{S}_2 \cdot \vec{v}_1 + 72 \hat{n} \cdot \vec{S}_1 \hat{n} \cdot \vec{S}_2 (\hat{n} \cdot \vec{v}_1)^2 - 5 \vec{S}_1 \cdot \vec{S}_2 (\hat{n} \cdot \vec{v}_1)^2 + 72 \hat{n} \cdot \vec{S}_1 \hat{n} \cdot \vec{S}_2 \hat{n} \cdot \vec{v}_2 \hat{n} \cdot \vec{v}_1 - \right. \right. \\ \left. \left. 3 \vec{S}_1 \cdot \vec{S}_2 \hat{n} \cdot \vec{v}_2 \hat{n} \cdot \vec{v}_1 - 24 \hat{n} \cdot \vec{S}_2 \hat{n} \cdot \vec{v}_1 \vec{S}_1 \cdot \vec{v}_1 - 12 \hat{n} \cdot \vec{S}_2 \hat{n} \cdot \vec{v}_1 \vec{S}_1 \cdot \vec{v}_2 - 19 \hat{n} \cdot \vec{S}_1 \hat{n} \cdot \vec{v}_1 \vec{S}_2 \cdot \vec{v}_1 - \right. \right. \\ \left. \left. 12 \hat{n} \cdot \vec{S}_1 \hat{n} \cdot \vec{v}_1 \vec{S}_2 \cdot \vec{v}_2 - 12 \hat{n} \cdot \vec{S}_2 \hat{n} \cdot \vec{v}_2 \vec{S}_1 \cdot \vec{v}_1 - 9 \hat{n} \cdot \vec{S}_1 \hat{n} \cdot \vec{v}_2 \vec{S}_2 \cdot \vec{v}_1 - 12 \vec{v}_1 \cdot \vec{v}_1 \hat{n} \cdot \vec{S}_1 \hat{n} \cdot \vec{S}_2 - \right. \right. \\ \left. \left. 12 \vec{v}_1 \cdot \vec{v}_2 \hat{n} \cdot \vec{S}_1 \hat{n} \cdot \vec{S}_2 + 3 \vec{S}_1 \cdot \vec{v}_1 \vec{S}_2 \cdot \vec{v}_1 + 2 \vec{S}_1 \cdot \vec{v}_2 \vec{S}_2 \cdot \vec{v}_1 + 3 \vec{S}_1 \cdot \vec{v}_1 \vec{S}_2 \cdot \vec{v}_2 + 3 \vec{S}_1 \cdot \vec{S}_2 \vec{v}_1 \cdot \vec{v}_1 + \vec{S}_1 \cdot \vec{S}_2 \vec{v}_1 \cdot \vec{v}_2 \right) \right) \}$$

{DiagS1S2 [3, 6, 10],

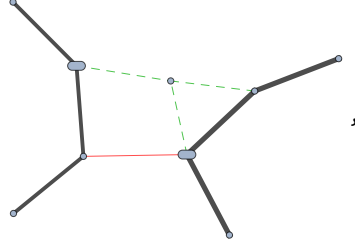

$$G^3 m_1 m_2 \left( \frac{1}{r^4} \left( 4 \vec{S}_1 \cdot \vec{S}_2 \hat{n} \cdot \vec{a}_1 - 4 \vec{S}_2 \cdot \vec{a}_1 \hat{n} \cdot \vec{S}_1 + 48 \hat{n} \cdot \vec{S}_2 \hat{n} \cdot \vec{S}_1 \hat{n} \cdot \vec{v}_1 - 64 \hat{n} \cdot \vec{S}_1 \hat{n} \cdot \vec{S}_2 \hat{n} \cdot \vec{v}_1 - 4 \vec{S}_1 \cdot \vec{S}_2 \hat{n} \cdot \vec{v}_1 - 4 \vec{S}_1 \cdot \vec{S}_2 \hat{n} \cdot \vec{v}_1 + 16 \hat{n} \cdot \vec{S}_2 \vec{S}_1 \cdot \vec{v}_1 - 8 \hat{n} \cdot \vec{S}_1 \vec{S}_2 \cdot \vec{v}_1 - 12 \hat{n} \cdot \vec{S}_2 \vec{S}_1 \cdot \vec{v}_1 + 20 \hat{n} \cdot \vec{S}_1 \vec{S}_2 \cdot \vec{v}_1 \right) + \frac{1}{r^5} \left( -32 \hat{n} \times \vec{S}_1 \cdot \vec{v}_1 \hat{n} \times \vec{S}_2 \cdot \vec{v}_1 + 352 \hat{n} \cdot \vec{S}_1 \hat{n} \cdot \vec{S}_2 (\hat{n} \cdot \vec{v}_1)^2 - 12 \vec{S}_1 \cdot \vec{S}_2 (\hat{n} \cdot \vec{v}_1)^2 + 224 \hat{n} \cdot \vec{S}_1 \hat{n} \cdot \vec{S}_2 \hat{n} \cdot \vec{v}_2 \hat{n} \cdot \vec{v}_1 - 20 \vec{S}_1 \cdot \vec{S}_2 \hat{n} \cdot \vec{v}_2 \hat{n} \cdot \vec{v}_1 - 112 \hat{n} \cdot \vec{S}_2 \hat{n} \cdot \vec{v}_1 \vec{S}_1 \cdot \vec{v}_1 - 48 \hat{n} \cdot \vec{S}_2 \hat{n} \cdot \vec{v}_1 \vec{S}_1 \cdot \vec{v}_2 - 100 \hat{n} \cdot \vec{S}_1 \hat{n} \cdot \vec{v}_1 \vec{S}_2 \cdot \vec{v}_1 - 48 \hat{n} \cdot \vec{S}_1 \hat{n} \cdot \vec{v}_1 \vec{S}_2 \cdot \vec{v}_2 - 32 \hat{n} \cdot \vec{S}_2 \hat{n} \cdot \vec{v}_2 \vec{S}_1 \cdot \vec{v}_1 - 12 \hat{n} \cdot \vec{S}_1 \hat{n} \cdot \vec{v}_2 \vec{S}_2 \cdot \vec{v}_1 - 48 \vec{v}_1 \cdot \vec{v}_1 \hat{n} \cdot \vec{S}_1 \hat{n} \cdot \vec{S}_2 - 48 \vec{v}_1 \cdot \vec{v}_2 \hat{n} \cdot \vec{S}_1 \hat{n} \cdot \vec{S}_2 + 12 \vec{S}_1 \cdot \vec{v}_1 \vec{S}_2 \cdot \vec{v}_1 + 8 \vec{S}_1 \cdot \vec{v}_2 \vec{S}_2 \cdot \vec{v}_1 + 12 \vec{S}_1 \cdot \vec{v}_1 \vec{S}_2 \cdot \vec{v}_2 + 12 \vec{S}_1 \cdot \vec{S}_2 \vec{v}_1 \cdot \vec{v}_1 + 4 \vec{S}_1 \cdot \vec{S}_2 \vec{v}_1 \cdot \vec{v}_2 \right) \right) \Bigg\}$$

{DiagS1S2 [3, 6, 11],

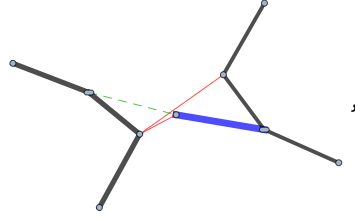

$$G^3 m_1 m_2 \left( \frac{1}{r^5} \left( 12 \hat{n} \cdot \vec{S}_1 \hat{n} \cdot \vec{S}_2 (\hat{n} \cdot \vec{v}_2)^2 - 12 \hat{n} \cdot \vec{S}_1 \hat{n} \cdot \vec{S}_2 \hat{n} \cdot \vec{v}_1 \hat{n} \cdot \vec{v}_2 - 4 \vec{S}_1 \cdot \vec{S}_2 \hat{n} \cdot \vec{v}_1 \hat{n} \cdot \vec{v}_2 - 3 \hat{n} \cdot \vec{S}_2 \hat{n} \cdot \vec{v}_2 \vec{S}_1 \cdot \vec{v}_2 + 4 \hat{n} \cdot \vec{S}_1 \hat{n} \cdot \vec{v}_2 \vec{S}_2 \cdot \vec{v}_1 - 3 \hat{n} \cdot \vec{S}_1 \hat{n} \cdot \vec{v}_2 \vec{S}_2 \cdot \vec{v}_2 + 3 \hat{n} \cdot \vec{S}_2 \hat{n} \cdot \vec{v}_1 \vec{S}_1 \cdot \vec{v}_2 + 3 \hat{n} \cdot \vec{S}_1 \hat{n} \cdot \vec{v}_1 \vec{S}_2 \cdot \vec{v}_2 - \vec{S}_1 \cdot \vec{v}_2 \vec{S}_2 \cdot \vec{v}_1 + \vec{S}_1 \cdot \vec{S}_2 \vec{v}_1 \cdot \vec{v}_2 \right) + \frac{-4 \hat{n} \cdot \vec{S}_1 \hat{n} \cdot \vec{S}_2 \hat{n} \cdot \vec{v}_2 + \hat{n} \cdot \vec{S}_2 \vec{S}_1 \cdot \vec{v}_2 + \hat{n} \cdot \vec{S}_1 \vec{S}_2 \cdot \vec{v}_2}{r^4} \right) \Bigg\}$$

{DiagS1S2 [3, 6, 12],

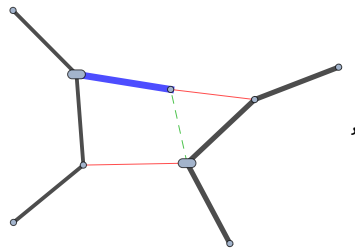

$$G^3 m_1 m_2 \left( \frac{1}{r^5} \left( -16 \hat{n} \cdot \vec{S}_1 \hat{n} \cdot \vec{S}_2 (\hat{n} \cdot \vec{v}_2)^2 + 16 \hat{n} \cdot \vec{S}_1 \hat{n} \cdot \vec{S}_2 \hat{n} \cdot \vec{v}_1 \hat{n} \cdot \vec{v}_2 - 16 \vec{S}_1 \cdot \vec{S}_2 \hat{n} \cdot \vec{v}_1 \hat{n} \cdot \vec{v}_2 + 4 \hat{n} \cdot \vec{S}_2 \hat{n} \cdot \vec{v}_2 \vec{S}_1 \cdot \vec{v}_2 + 16 \hat{n} \cdot \vec{S}_1 \hat{n} \cdot \vec{v}_2 \vec{S}_2 \cdot \vec{v}_1 + 4 \hat{n} \cdot \vec{S}_1 \hat{n} \cdot \vec{v}_2 \vec{S}_2 \cdot \vec{v}_2 - 4 \hat{n} \cdot \vec{S}_2 \hat{n} \cdot \vec{v}_1 \vec{S}_1 \cdot \vec{v}_2 - 4 \hat{n} \cdot \vec{S}_1 \hat{n} \cdot \vec{v}_1 \vec{S}_2 \cdot \vec{v}_2 - 4 \vec{S}_1 \cdot \vec{v}_2 \vec{S}_2 \cdot \vec{v}_1 + 4 \vec{S}_1 \cdot \vec{S}_2 \vec{v}_1 \cdot \vec{v}_2 \right) + \frac{-16 \hat{n} \cdot \vec{S}_1 \hat{n} \cdot \vec{S}_2 \hat{n} \cdot \vec{v}_2 + 4 \hat{n} \cdot \vec{S}_2 \vec{S}_1 \cdot \vec{v}_2 + 4 \hat{n} \cdot \vec{S}_1 \vec{S}_2 \cdot \vec{v}_2}{r^4} \right) \Bigg\}$$



{DiagS1S2 [3, 6, 13],

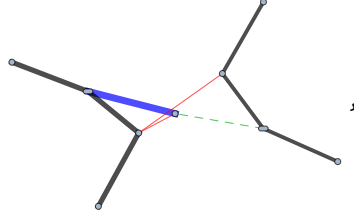

,

$$G^3 m_1 m_2 \left\{ \frac{1}{r^5} \left( -4 \hat{n} \times \vec{S}_1 \cdot \vec{v}_1 \hat{n} \times \vec{S}_2 \cdot \vec{v}_1 + 40 \hat{n} \cdot \vec{S}_1 \hat{n} \cdot \vec{S}_2 (\hat{n} \cdot \vec{v}_1)^2 + 4 \vec{S}_1 \cdot \vec{S}_2 (\hat{n} \cdot \vec{v}_1)^2 - 40 \hat{n} \cdot \vec{S}_1 \hat{n} \cdot \vec{S}_2 \hat{n} \cdot \vec{v}_2 \hat{n} \cdot \vec{v}_1 - \right. \right. \\ \left. \left. 4 \vec{S}_1 \cdot \vec{S}_2 \hat{n} \cdot \vec{v}_2 \hat{n} \cdot \vec{v}_1 - 12 \hat{n} \cdot \vec{S}_2 \hat{n} \cdot \vec{v}_1 \vec{S}_1 \cdot \vec{v}_1 + 4 \hat{n} \cdot \vec{S}_2 \hat{n} \cdot \vec{v}_1 \vec{S}_1 \cdot \vec{v}_2 - 16 \hat{n} \cdot \vec{S}_1 \hat{n} \cdot \vec{v}_1 \vec{S}_2 \cdot \vec{v}_1 + \right. \right. \\ \left. \left. 4 \hat{n} \cdot \vec{S}_1 \hat{n} \cdot \vec{v}_1 \vec{S}_2 \cdot \vec{v}_2 + 8 \hat{n} \cdot \vec{S}_2 \hat{n} \cdot \vec{v}_2 \vec{S}_1 \cdot \vec{v}_1 + 12 \hat{n} \cdot \vec{S}_1 \hat{n} \cdot \vec{v}_2 \vec{S}_2 \cdot \vec{v}_1 - 4 \vec{v}_1 \cdot \vec{v}_1 \hat{n} \cdot \vec{S}_1 \hat{n} \cdot \vec{S}_2 + \right. \right. \\ \left. \left. 4 \vec{v}_1 \cdot \vec{v}_2 \hat{n} \cdot \vec{S}_1 \hat{n} \cdot \vec{S}_2 + 2 \vec{S}_1 \cdot \vec{v}_1 \vec{S}_2 \cdot \vec{v}_1 - 2 \vec{S}_1 \cdot \vec{v}_2 \vec{S}_2 \cdot \vec{v}_1 - \vec{S}_1 \cdot \vec{v}_1 \vec{S}_2 \cdot \vec{v}_2 + \vec{S}_1 \cdot \vec{S}_2 \vec{v}_1 \cdot \vec{v}_2 \right) + \right. \\ \left. \frac{-4 \hat{n} \cdot \vec{S}_2 \hat{n} \cdot \vec{S}_1 \hat{n} \cdot \vec{v}_1 - \vec{S}_1 \cdot \vec{S}_2 \hat{n} \cdot \vec{v}_1 + 2 \hat{n} \cdot \vec{S}_1 \vec{S}_2 \cdot \vec{v}_1 + \hat{n} \cdot \vec{S}_2 \vec{S}_1 \cdot \vec{v}_1}{r^4} \right\}$$

{DiagS1S2 [3, 6, 14],

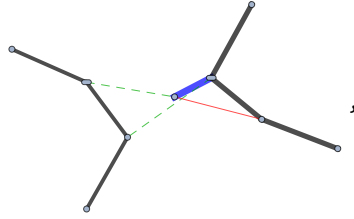

,

$$G^3 m_1 m_2 \left\{ \frac{1}{r^5} \left( 8 \hat{n} \times \vec{S}_1 \cdot \vec{v}_2 \hat{n} \times \vec{S}_2 \cdot \vec{v}_1 - 8 \hat{n} \times \vec{S}_1 \cdot \vec{v}_1 \hat{n} \times \vec{S}_2 \cdot \vec{v}_2 + 32 \hat{n} \cdot \vec{S}_1 \hat{n} \cdot \vec{S}_2 (\hat{n} \cdot \vec{v}_2)^2 - 32 \hat{n} \cdot \vec{S}_1 \hat{n} \cdot \vec{S}_2 \hat{n} \cdot \vec{v}_1 \hat{n} \cdot \vec{v}_2 + \right. \right. \\ \left. \left. 8 \hat{n} \cdot \vec{S}_2 \hat{n} \cdot \vec{v}_2 \vec{S}_1 \cdot \vec{v}_1 - 8 \hat{n} \cdot \vec{S}_2 \hat{n} \cdot \vec{v}_2 \vec{S}_1 \cdot \vec{v}_2 - 24 \hat{n} \cdot \vec{S}_1 \hat{n} \cdot \vec{v}_2 \vec{S}_2 \cdot \vec{v}_2 + 24 \hat{n} \cdot \vec{S}_1 \hat{n} \cdot \vec{v}_1 \vec{S}_2 \cdot \vec{v}_2 + 8 \vec{v}_1 \cdot \vec{v}_2 \hat{n} \cdot \vec{S}_1 \hat{n} \cdot \vec{S}_2 - \right. \right. \\ \left. \left. 8 \vec{v}_2 \cdot \vec{v}_2 \hat{n} \cdot \vec{S}_1 \hat{n} \cdot \vec{S}_2 - 8 \vec{S}_1 \cdot \vec{v}_1 \vec{S}_2 \cdot \vec{v}_2 + 8 \vec{S}_1 \cdot \vec{v}_2 \vec{S}_2 \cdot \vec{v}_2 \right) + \frac{8 \hat{n} \cdot \vec{S}_2 \hat{n} \cdot \vec{S}_1 \hat{n} \cdot \vec{v}_2 - 8 \hat{n} \cdot \vec{S}_1 \vec{S}_2 \cdot \vec{v}_2}{r^4} \right\}$$

{DiagS1S2 [3, 6, 15],

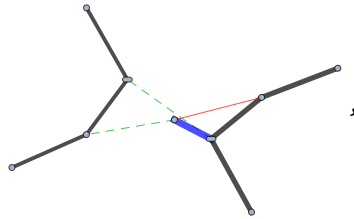

,

$$G^3 m_1 m_2 \left\{ \frac{12 \hat{n} \cdot \vec{a}_2 \hat{n} \cdot \vec{S}_1 \hat{n} \cdot \vec{S}_2 - 8 \vec{S}_1 \cdot \vec{a}_2 \hat{n} \cdot \vec{S}_2 - 8 \vec{S}_1 \cdot \vec{S}_2 \hat{n} \cdot \vec{a}_2 + 4 \vec{S}_2 \cdot \vec{a}_2 \hat{n} \cdot \vec{S}_1}{r^4} + \frac{1}{r^5} \right. \\ \left. \left( -12 \hat{n} \times \vec{S}_1 \cdot \vec{v}_2 \hat{n} \times \vec{S}_2 \cdot \vec{v}_1 - 12 \hat{n} \times \vec{S}_1 \cdot \vec{v}_1 \hat{n} \times \vec{S}_2 \cdot \vec{v}_2 + 24 \hat{n} \times \vec{S}_1 \cdot \vec{v}_2 \hat{n} \times \vec{S}_2 \cdot \vec{v}_2 + 24 \hat{n} \cdot \vec{S}_1 \hat{n} \cdot \vec{S}_2 (\hat{n} \cdot \vec{v}_2)^2 + \right. \right. \\ \left. \left. 8 \vec{S}_1 \cdot \vec{S}_2 (\hat{n} \cdot \vec{v}_2)^2 - 24 \hat{n} \cdot \vec{S}_1 \hat{n} \cdot \vec{S}_2 \hat{n} \cdot \vec{v}_1 \hat{n} \cdot \vec{v}_2 - 8 \vec{S}_1 \cdot \vec{S}_2 \hat{n} \cdot \vec{v}_1 \hat{n} \cdot \vec{v}_2 - 16 \hat{n} \cdot \vec{S}_2 \hat{n} \cdot \vec{v}_2 \vec{S}_1 \cdot \vec{v}_2 + \right. \right. \\ \left. \left. 12 \hat{n} \cdot \vec{S}_1 \hat{n} \cdot \vec{v}_2 \vec{S}_2 \cdot \vec{v}_1 - 16 \hat{n} \cdot \vec{S}_1 \hat{n} \cdot \vec{v}_2 \vec{S}_2 \cdot \vec{v}_2 + 16 \hat{n} \cdot \vec{S}_2 \hat{n} \cdot \vec{v}_1 \vec{S}_1 \cdot \vec{v}_2 + 4 \hat{n} \cdot \vec{S}_1 \hat{n} \cdot \vec{v}_1 \vec{S}_2 \cdot \vec{v}_2 - \right. \right. \\ \left. \left. 8 \vec{S}_1 \cdot \vec{v}_2 \vec{S}_2 \cdot \vec{v}_1 - 8 \vec{S}_1 \cdot \vec{v}_1 \vec{S}_2 \cdot \vec{v}_2 + 16 \vec{S}_1 \cdot \vec{v}_2 \vec{S}_2 \cdot \vec{v}_2 + 16 \vec{S}_1 \cdot \vec{S}_2 \vec{v}_1 \cdot \vec{v}_2 - 16 \vec{S}_1 \cdot \vec{S}_2 \vec{v}_2 \cdot \vec{v}_2 \right) \right\}$$

{DiagS1S2 [3, 6, 16],

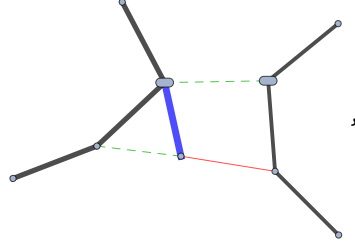

,

$$G^3 m_1 m_2 \left( \frac{-24 \hat{n} \cdot \vec{a}_1 \hat{n} \cdot \vec{S}_1 \hat{n} \cdot \vec{S}_2 + 16 \vec{S}_1 \cdot \vec{a}_1 \hat{n} \cdot \vec{S}_2 + 16 \vec{S}_1 \cdot \vec{S}_2 \hat{n} \cdot \vec{a}_1 - 8 \vec{S}_2 \cdot \vec{a}_1 \hat{n} \cdot \vec{S}_1}{r^4} + \frac{1}{r^5} \right. \\ \left. \left( 24 \hat{n} \times \vec{S}_1 \cdot \vec{v}_1 \hat{n} \times \vec{S}_2 \cdot \vec{v}_1 - 12 \hat{n} \times \vec{S}_1 \cdot \vec{v}_2 \hat{n} \times \vec{S}_2 \cdot \vec{v}_1 - 12 \hat{n} \times \vec{S}_1 \cdot \vec{v}_1 \hat{n} \times \vec{S}_2 \cdot \vec{v}_2 + 24 \hat{n} \cdot \vec{S}_1 \hat{n} \cdot \vec{S}_2 (\hat{n} \cdot \vec{v}_1)^2 + \right. \right. \\ \left. \left. 8 \vec{S}_1 \cdot \vec{S}_2 (\hat{n} \cdot \vec{v}_1)^2 - 24 \hat{n} \cdot \vec{S}_1 \hat{n} \cdot \vec{S}_2 \hat{n} \cdot \vec{v}_2 \hat{n} \cdot \vec{v}_1 - 8 \vec{S}_1 \cdot \vec{S}_2 \hat{n} \cdot \vec{v}_2 \hat{n} \cdot \vec{v}_1 - 16 \hat{n} \cdot \vec{S}_2 \hat{n} \cdot \vec{v}_1 \vec{S}_1 \cdot \vec{v}_1 - \right. \right. \\ \left. \left. 16 \hat{n} \cdot \vec{S}_1 \hat{n} \cdot \vec{v}_1 \vec{S}_2 \cdot \vec{v}_1 + 12 \hat{n} \cdot \vec{S}_1 \hat{n} \cdot \vec{v}_1 \vec{S}_2 \cdot \vec{v}_2 + 16 \hat{n} \cdot \vec{S}_2 \hat{n} \cdot \vec{v}_2 \vec{S}_1 \cdot \vec{v}_1 + 4 \hat{n} \cdot \vec{S}_1 \hat{n} \cdot \vec{v}_2 \vec{S}_2 \cdot \vec{v}_1 + \right. \right. \\ \left. \left. 16 \vec{S}_1 \cdot \vec{v}_1 \vec{S}_2 \cdot \vec{v}_1 - 8 \vec{S}_1 \cdot \vec{v}_2 \vec{S}_2 \cdot \vec{v}_1 - 8 \vec{S}_1 \cdot \vec{v}_1 \vec{S}_2 \cdot \vec{v}_2 - 16 \vec{S}_1 \cdot \vec{S}_2 \vec{v}_1 \cdot \vec{v}_1 + 16 \vec{S}_1 \cdot \vec{S}_2 \vec{v}_1 \cdot \vec{v}_2 \right) \right) \Bigg\}$$

{DiagS1S2 [3, 6, 17],

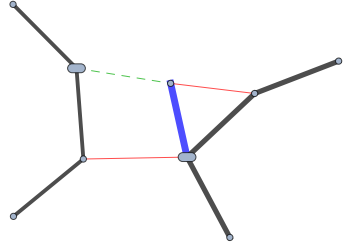

,

$$G^3 m_1 m_2 \left( \frac{1}{r^5} \left( -16 \hat{n} \times \vec{S}_1 \cdot \vec{v}_1 \hat{n} \times \vec{S}_2 \cdot \vec{v}_1 + 8 \hat{n} \times \vec{S}_1 \cdot \vec{v}_2 \hat{n} \times \vec{S}_2 \cdot \vec{v}_1 + 8 \hat{n} \times \vec{S}_1 \cdot \vec{v}_1 \hat{n} \times \vec{S}_2 \cdot \vec{v}_2 - 32 \hat{n} \cdot \vec{S}_1 \hat{n} \cdot \vec{S}_2 (\hat{n} \cdot \vec{v}_1)^2 + \right. \right. \\ \left. \left. 48 \vec{S}_1 \cdot \vec{S}_2 (\hat{n} \cdot \vec{v}_1)^2 + 32 \hat{n} \cdot \vec{S}_1 \hat{n} \cdot \vec{S}_2 \hat{n} \cdot \vec{v}_2 \hat{n} \cdot \vec{v}_1 - 48 \vec{S}_1 \cdot \vec{S}_2 \hat{n} \cdot \vec{v}_2 \hat{n} \cdot \vec{v}_1 + 8 \hat{n} \cdot \vec{S}_2 \hat{n} \cdot \vec{v}_1 \vec{S}_1 \cdot \vec{v}_1 - \right. \right. \\ \left. \left. 8 \hat{n} \cdot \vec{S}_2 \hat{n} \cdot \vec{v}_1 \vec{S}_1 \cdot \vec{v}_2 - 24 \hat{n} \cdot \vec{S}_1 \hat{n} \cdot \vec{v}_1 \vec{S}_2 \cdot \vec{v}_1 + 24 \hat{n} \cdot \vec{S}_1 \hat{n} \cdot \vec{v}_2 \vec{S}_2 \cdot \vec{v}_1 + 8 \vec{v}_1 \cdot \vec{v}_1 \hat{n} \cdot \vec{S}_1 \hat{n} \cdot \vec{S}_2 - \right. \right. \\ \left. \left. 8 \vec{v}_1 \cdot \vec{v}_2 \hat{n} \cdot \vec{S}_1 \hat{n} \cdot \vec{S}_2 + 8 \vec{S}_1 \cdot \vec{v}_1 \vec{S}_2 \cdot \vec{v}_1 - 8 \vec{S}_1 \cdot \vec{v}_2 \vec{S}_2 \cdot \vec{v}_1 - 16 \vec{S}_1 \cdot \vec{S}_2 \vec{v}_1 \cdot \vec{v}_1 + 16 \vec{S}_1 \cdot \vec{S}_2 \vec{v}_1 \cdot \vec{v}_2 \right) + \right. \\ \left. \frac{8 \hat{n} \cdot \vec{S}_2 \hat{n} \cdot \vec{S}_1 \hat{n} \cdot \vec{v}_1 - 16 \vec{S}_1 \cdot \vec{S}_2 \hat{n} \cdot \vec{v}_1 + 8 \hat{n} \cdot \vec{S}_1 \vec{S}_2 \cdot \vec{v}_1}{r^4} \right) \Bigg\}$$

{DiagS1S2 [3, 6, 18],

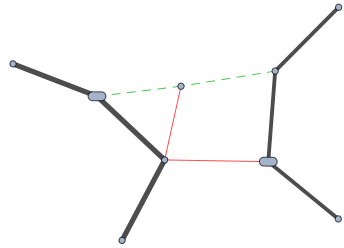

$$, - \frac{4 G^3 m_1 m_2 \hat{n} \times \vec{S}_1 \cdot \vec{v}_2 \hat{n} \times \vec{S}_2 \cdot \vec{v}_2}{r^5} \Bigg\}$$

{DiagS1S2 [3, 6, 19],

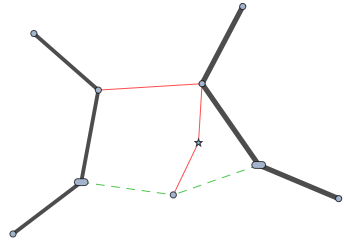

,

$$G^3 m_1 m_2 \left( \frac{1}{r^5} \left( 2 \hat{n} \times \vec{S}_1 \cdot \vec{v}_1 \hat{n} \times \vec{S}_2 \cdot \vec{v}_1 + 6 \hat{n} \cdot \vec{S}_1 \hat{n} \cdot \vec{S}_2 (\hat{n} \cdot \vec{v}_1)^2 - \frac{1}{2} \vec{S}_1 \cdot \vec{S}_2 (\hat{n} \cdot \vec{v}_1)^2 - 4 \hat{n} \cdot \vec{S}_1 \hat{n} \cdot \vec{S}_2 \hat{n} \cdot \vec{v}_2 \hat{n} \cdot \vec{v}_1 + \right. \right. \\ \left. \frac{9}{2} \vec{S}_1 \cdot \vec{S}_2 \hat{n} \cdot \vec{v}_2 \hat{n} \cdot \vec{v}_1 - 3 \hat{n} \cdot \vec{S}_2 \hat{n} \cdot \vec{v}_1 \vec{S}_1 \cdot \vec{v}_1 + 2 \hat{n} \cdot \vec{S}_2 \hat{n} \cdot \vec{v}_1 \vec{S}_1 \cdot \vec{v}_2 - \frac{5}{2} \hat{n} \cdot \vec{S}_1 \hat{n} \cdot \vec{v}_1 \vec{S}_2 \cdot \vec{v}_1 + 2 \hat{n} \cdot \vec{S}_1 \hat{n} \cdot \vec{v}_1 \vec{S}_2 \cdot \vec{v}_2 - \right. \\ \left. 8 \hat{n} \cdot \vec{S}_1 \hat{n} \cdot \vec{S}_2 (\hat{n} \cdot \vec{v}_2)^2 + \hat{n} \cdot \vec{S}_2 \hat{n} \cdot \vec{v}_2 \vec{S}_1 \cdot \vec{v}_1 + 2 \hat{n} \cdot \vec{S}_2 \hat{n} \cdot \vec{v}_2 \vec{S}_1 \cdot \vec{v}_2 - \frac{7}{2} \hat{n} \cdot \vec{S}_1 \hat{n} \cdot \vec{v}_2 \vec{S}_2 \cdot \vec{v}_1 + 2 \hat{n} \cdot \vec{S}_1 \hat{n} \cdot \vec{v}_2 \vec{S}_2 \cdot \vec{v}_2 + \right. \\ \left. 4 \vec{v}_1 \cdot \vec{v}_2 \hat{n} \cdot \vec{S}_1 \hat{n} \cdot \vec{S}_2 + \frac{3}{2} \vec{S}_1 \cdot \vec{v}_1 \vec{S}_2 \cdot \vec{v}_1 + \frac{1}{2} \vec{S}_1 \cdot \vec{v}_2 \vec{S}_2 \cdot \vec{v}_1 - \vec{S}_1 \cdot \vec{v}_1 \vec{S}_2 \cdot \vec{v}_2 - \frac{3}{2} \vec{S}_1 \cdot \vec{S}_2 \vec{v}_1 \cdot \vec{v}_1 - \frac{3}{2} \vec{S}_1 \cdot \vec{S}_2 \vec{v}_1 \cdot \vec{v}_2 \right) + \\ \left. \frac{1}{r^4} \left( -2 \hat{n} \cdot \vec{S}_2 \hat{n} \cdot \vec{S}_1 \hat{n} \cdot \vec{v}_1 - 2 \hat{n} \cdot \vec{S}_1 \hat{n} \cdot \vec{S}_2 \hat{n} \cdot \vec{v}_1 + \frac{3}{2} \vec{S}_1 \cdot \vec{S}_2 \hat{n} \cdot \vec{v}_1 + \frac{3}{2} \vec{S}_1 \cdot \vec{S}_2 \hat{n} \cdot \vec{v}_1 - 2 \hat{n} \cdot \vec{S}_2 \hat{n} \cdot \vec{S}_1 \hat{n} \cdot \vec{v}_2 - \right. \right. \\ \left. \left. 2 \hat{n} \cdot \vec{S}_1 \hat{n} \cdot \vec{S}_2 \hat{n} \cdot \vec{v}_2 + \hat{n} \cdot \vec{S}_2 \vec{S}_1 \cdot \vec{v}_1 - \frac{1}{2} \hat{n} \cdot \vec{S}_1 \vec{S}_2 \cdot \vec{v}_1 + \hat{n} \cdot \vec{S}_2 \vec{S}_1 \cdot \vec{v}_1 - \frac{1}{2} \hat{n} \cdot \vec{S}_1 \vec{S}_2 \cdot \vec{v}_1 \right) \right) \Bigg\}$$

{DiagS1S2 [3, 6, 20],

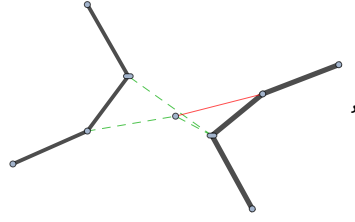

$$G^3 m_1 m_2 \left( \frac{-8 \vec{S}_1 \cdot \vec{S}_2 \hat{n} \cdot \vec{a}_2 + 8 \vec{S}_2 \cdot \vec{a}_2 \hat{n} \cdot \vec{S}_1 - 8 \hat{n} \cdot \vec{S}_1 \vec{S}_2 \cdot \vec{v}_2 + 8 \vec{S}_1 \cdot \vec{S}_2 \hat{n} \cdot \vec{v}_2}{r^4} + \frac{1}{r^5} \right. \\ \left. \left( 4 \hat{n} \times \vec{S}_1 \cdot \vec{v}_2 \hat{n} \times \vec{S}_2 \cdot \vec{v}_1 + 8 \vec{S}_1 \cdot \vec{S}_2 (\hat{n} \cdot \vec{v}_2)^2 + 12 \vec{S}_1 \cdot \vec{S}_2 \hat{n} \cdot \vec{v}_1 \hat{n} \cdot \vec{v}_2 - 4 \hat{n} \cdot \vec{S}_1 \hat{n} \cdot \vec{v}_2 \vec{S}_2 \cdot \vec{v}_1 - 8 \hat{n} \cdot \vec{S}_1 \hat{n} \cdot \vec{v}_2 \vec{S}_2 \cdot \vec{v}_2 - \right. \right. \\ \left. \left. 8 \hat{n} \cdot \vec{S}_1 \hat{n} \cdot \vec{v}_1 \vec{S}_2 \cdot \vec{v}_2 - 20 \vec{v}_1 \cdot \vec{v}_2 \hat{n} \cdot \vec{S}_1 \hat{n} \cdot \vec{S}_2 + 8 \vec{S}_1 \cdot \vec{v}_2 \vec{S}_2 \cdot \vec{v}_2 + 4 \vec{S}_1 \cdot \vec{S}_2 \vec{v}_1 \cdot \vec{v}_2 - 8 \vec{S}_1 \cdot \vec{S}_2 \vec{v}_2 \cdot \vec{v}_2 \right) \right) \Bigg\}$$

{DiagS1S2 [3, 6, 21],

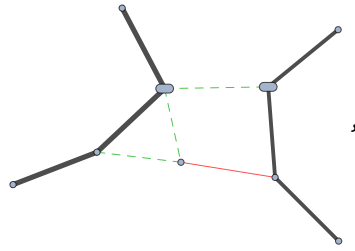

$$G^3 m_1 m_2 \left( \frac{8 \vec{S}_1 \cdot \vec{S}_2 \hat{n} \cdot \vec{a}_1 - 8 \vec{S}_2 \cdot \vec{a}_1 \hat{n} \cdot \vec{S}_1 + 8 \hat{n} \cdot \vec{S}_1 \vec{S}_2 \cdot \vec{v}_1 - 8 \vec{S}_1 \cdot \vec{S}_2 \hat{n} \cdot \vec{v}_1}{r^4} + \frac{1}{r^5} \right. \\ \left. \left( -4 \hat{n} \times \vec{S}_1 \cdot \vec{v}_1 \hat{n} \times \vec{S}_2 \cdot \vec{v}_1 - 12 \vec{S}_1 \cdot \vec{S}_2 (\hat{n} \cdot \vec{v}_1)^2 - 8 \vec{S}_1 \cdot \vec{S}_2 \hat{n} \cdot \vec{v}_2 \hat{n} \cdot \vec{v}_1 + 12 \hat{n} \cdot \vec{S}_1 \hat{n} \cdot \vec{v}_1 \vec{S}_2 \cdot \vec{v}_1 + \right. \right. \\ \left. \left. 8 \hat{n} \cdot \vec{S}_1 \hat{n} \cdot \vec{v}_2 \vec{S}_2 \cdot \vec{v}_1 + 20 \vec{v}_1 \cdot \vec{v}_1 \hat{n} \cdot \vec{S}_1 \hat{n} \cdot \vec{S}_2 - 8 \vec{S}_1 \cdot \vec{v}_2 \vec{S}_2 \cdot \vec{v}_1 - 4 \vec{S}_1 \cdot \vec{S}_2 \vec{v}_1 \cdot \vec{v}_1 + 8 \vec{S}_1 \cdot \vec{S}_2 \vec{v}_1 \cdot \vec{v}_2 \right) \right) \Bigg\}$$

{DiagS1S2 [3, 6, 22],

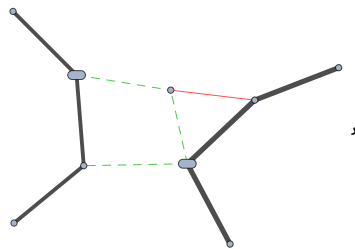

$$G^3 m_1 m_2 \left\{ \frac{-16 \vec{S}_1 \cdot \vec{S}_2 \hat{n} \cdot \vec{a}_2 + 16 \vec{S}_2 \cdot \vec{a}_2 \hat{n} \cdot \vec{S}_1 - 16 \hat{n} \cdot \vec{S}_1 \vec{S}_2 \cdot \vec{v}_2 + 16 \vec{S}_1 \cdot \vec{S}_2 \hat{n} \cdot \vec{v}_2}{r^4} + \frac{1}{r^5} \right. \\ \left. \left( 48 \vec{S}_1 \cdot \vec{S}_2 (\hat{n} \cdot \vec{v}_2)^2 - 32 \vec{S}_1 \cdot \vec{S}_2 \hat{n} \cdot \vec{v}_1 \hat{n} \cdot \vec{v}_2 - 48 \hat{n} \cdot \vec{S}_1 \hat{n} \cdot \vec{v}_2 \vec{S}_2 \cdot \vec{v}_2 + 32 \hat{n} \cdot \vec{S}_1 \hat{n} \cdot \vec{v}_1 \vec{S}_2 \cdot \vec{v}_2 - \right. \right. \\ \left. \left. 16 \vec{v}_1 \cdot \vec{v}_2 \hat{n} \cdot \vec{S}_1 \hat{n} \cdot \vec{S}_2 - 12 \vec{S}_1 \cdot \vec{v}_1 \vec{S}_2 \cdot \vec{v}_2 + 16 \vec{S}_1 \cdot \vec{v}_2 \vec{S}_2 \cdot \vec{v}_2 + 20 \vec{S}_1 \cdot \vec{S}_2 \vec{v}_1 \cdot \vec{v}_2 - 16 \vec{S}_1 \cdot \vec{S}_2 \vec{v}_2 \cdot \vec{v}_2 \right) \right\}$$

{DiagS1S2 [3, 6, 23],

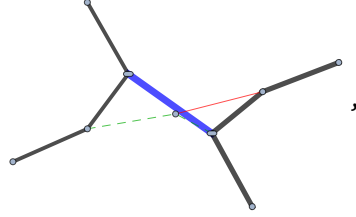

,

$$\frac{G^3 m_1 m_2 \left( 6 \hat{n} \times \vec{S}_1 \cdot \vec{v}_2 \hat{n} \times \vec{S}_2 \cdot \vec{v}_2 + 2 \vec{S}_1 \cdot \vec{S}_2 (\hat{n} \cdot \vec{v}_2)^2 - 2 \hat{n} \cdot \vec{S}_1 \hat{n} \cdot \vec{v}_2 \vec{S}_2 \cdot \vec{v}_2 + 2 \vec{v}_2 \cdot \vec{v}_2 \hat{n} \cdot \vec{S}_1 \hat{n} \cdot \vec{S}_2 - 2 \vec{S}_1 \cdot \vec{S}_2 \vec{v}_2 \cdot \vec{v}_2 \right)}{r^5}$$

{DiagS1S2 [3, 6, 24],

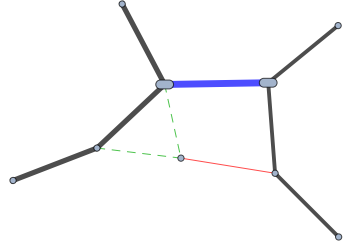

,  $\frac{1}{r^5}$

$$G^3 m_1 m_2 \left\{ 2 \hat{n} \times \vec{S}_1 \cdot \vec{v}_2 \hat{n} \times \vec{S}_2 \cdot \vec{v}_1 - 8 \hat{n} \times \vec{S}_1 \cdot \vec{v}_1 \hat{n} \times \vec{S}_2 \cdot \vec{v}_2 - 2 \vec{S}_1 \cdot \vec{S}_2 \hat{n} \cdot \vec{v}_1 \hat{n} \cdot \vec{v}_2 + \right. \\ \left. 2 \hat{n} \cdot \vec{S}_1 \hat{n} \cdot \vec{v}_2 \vec{S}_2 \cdot \vec{v}_1 - 2 \vec{v}_1 \cdot \vec{v}_2 \hat{n} \cdot \vec{S}_1 \hat{n} \cdot \vec{S}_2 + 2 \vec{S}_1 \cdot \vec{S}_2 \vec{v}_1 \cdot \vec{v}_2 \right\}$$

{DiagS1S2 [3, 6, 25],

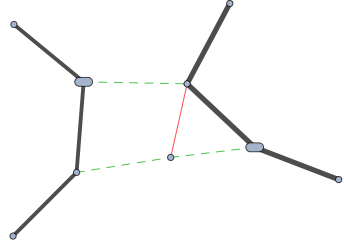

,  $\frac{4 G^3 m_1 m_2 \hat{n} \times \vec{S}_1 \cdot \vec{v}_2 \hat{n} \times \vec{S}_2 \cdot \vec{v}_1}{r^5}$

{DiagS1S2 [3, 6, 26],

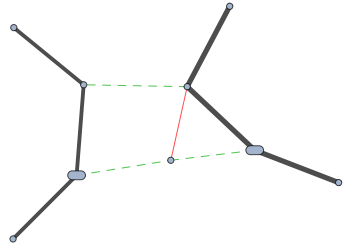

,  $\frac{G^3 m_1 m_2 \left( 8 \vec{S}_1 \cdot \vec{S}_2 \vec{v}_1 \cdot \vec{v}_2 - 16 \vec{v}_1 \cdot \vec{v}_2 \hat{n} \cdot \vec{S}_1 \hat{n} \cdot \vec{S}_2 \right)}{r^5}$

$\{\text{DiagS1S2}[3, 6, 27],$ 
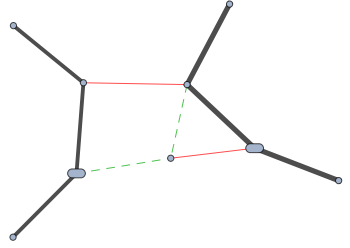
 $,$ 

$$\frac{G^3 m_1 m_2 \left( -32 \hat{n} \times \vec{S}_1 \cdot \vec{v}_1 \hat{n} \times \vec{S}_2 \cdot \vec{v}_1 - 16 \vec{S}_1 \cdot \vec{S}_2 (\hat{n} \cdot \vec{v}_1)^2 + 16 \hat{n} \cdot \vec{S}_1 \hat{n} \cdot \vec{v}_1 \vec{S}_2 \cdot \vec{v}_1 - 12 \vec{S}_1 \cdot \vec{v}_1 \vec{S}_2 \cdot \vec{v}_1 + 12 \vec{S}_1 \cdot \vec{S}_2 \vec{v}_1 \cdot \vec{v}_1 \right)}{r^5}$$

 $\{\text{DiagS1S2}[3, 6, 28],$ 
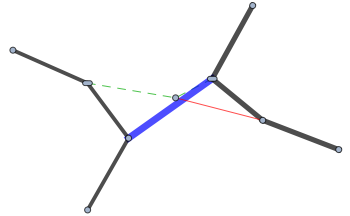
 $, \frac{1}{r^5}$ 

$$G^3 m_1 m_2 \left( -8 \hat{n} \times \vec{S}_1 \cdot \vec{v}_2 \hat{n} \times \vec{S}_2 \cdot \vec{v}_2 - 8 \vec{S}_1 \cdot \vec{S}_2 (\hat{n} \cdot \vec{v}_2)^2 + 8 \hat{n} \cdot \vec{S}_1 \hat{n} \cdot \vec{v}_2 \vec{S}_2 \cdot \vec{v}_2 - 16 \vec{v}_2 \cdot \vec{v}_2 \hat{n} \cdot \vec{S}_1 \hat{n} \cdot \vec{S}_2 - 4 \vec{S}_1 \cdot \vec{v}_2 \vec{S}_2 \cdot \vec{v}_2 + 12 \vec{S}_1 \cdot \vec{S}_2 \vec{v}_2 \cdot \vec{v}_2 \right)$$

 $\{\text{DiagS1S2}[3, 6, 29],$ 
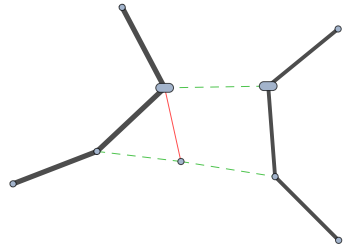

$$, \frac{G^3 m_1 m_2 \left( 32 \vec{S}_1 \cdot \vec{S}_2 \vec{v}_1 \cdot \vec{v}_2 - 96 \vec{v}_1 \cdot \vec{v}_2 \hat{n} \cdot \vec{S}_1 \hat{n} \cdot \vec{S}_2 \right)}{r^5}$$

 $\{\text{DiagS1S2}[3, 6, 30],$ 
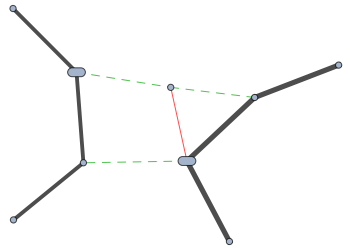

$$, \frac{64 G^3 m_1 m_2 \hat{n} \times \vec{S}_1 \cdot \vec{v}_2 \hat{n} \times \vec{S}_2 \cdot \vec{v}_1}{r^5}$$

 $\{\text{DiagS1S2}[3, 6, 31],$ 
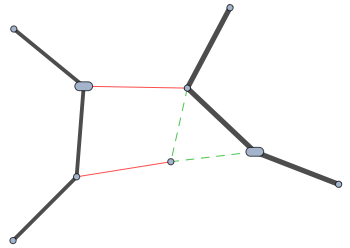

$$, \frac{4 G^3 m_1 m_2 \hat{n} \times \vec{S}_1 \cdot \vec{v}_1 \hat{n} \times \vec{S}_2 \cdot \vec{v}_2}{r^5}$$

 $\{\text{DiagS1S2}[3, 6, 32],$ 
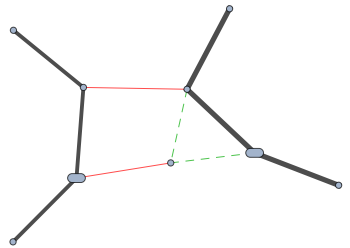
 $,$

$$\frac{G^3 m_1 m_2 \left( 16 \hat{n} \times \vec{S}_1 \cdot \vec{v}_1 \hat{n} \times \vec{S}_2 \cdot \vec{v}_2 + 4 \vec{S}_1 \cdot \vec{v}_2 \vec{S}_2 \cdot \vec{v}_1 - 4 \vec{S}_1 \cdot \vec{S}_2 \vec{v}_1 \cdot \vec{v}_2 \right)}{r^5} \}$$

{DiagS1S2 [3, 6, 33],

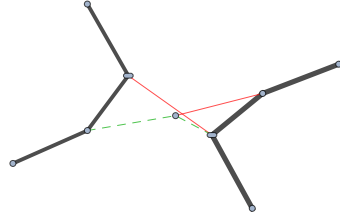

,  $-\frac{16 G^3 m_1 m_2 \hat{n} \times \vec{S}_1 \cdot \vec{v}_2 \hat{n} \times \vec{S}_2 \cdot \vec{v}_2}{r^5}$ }

{DiagS1S2 [3, 6, 34],

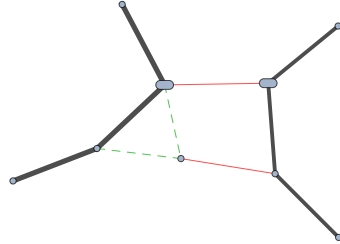

,  $\frac{16 G^3 m_1 m_2 \hat{n} \times \vec{S}_1 \cdot \vec{v}_1 \hat{n} \times \vec{S}_2 \cdot \vec{v}_2}{r^5}$ }

{DiagS1S2 [3, 6, 35],

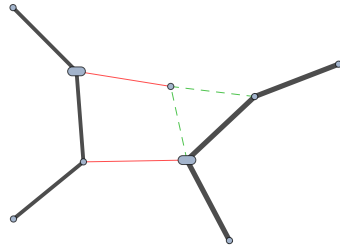

,

$$\frac{G^3 m_1 m_2 \left( 64 \hat{n} \times \vec{S}_1 \cdot \vec{v}_1 \hat{n} \times \vec{S}_2 \cdot \vec{v}_2 + 16 \vec{S}_1 \cdot \vec{v}_2 \vec{S}_2 \cdot \vec{v}_1 - 16 \vec{S}_1 \cdot \vec{S}_2 \vec{v}_1 \cdot \vec{v}_2 \right)}{r^5} \}$$

{DiagS1S2 [3, 6, 36],

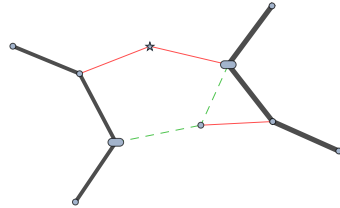

,

$$G^3 m_1 m_2 \left\{ \frac{1}{r^5} \left( 48 \hat{n} \cdot \vec{S}_1 \hat{n} \cdot \vec{S}_2 (\hat{n} \cdot \vec{v}_2)^2 - 16 \vec{S}_1 \cdot \vec{S}_2 (\hat{n} \cdot \vec{v}_2)^2 - 56 \hat{n} \cdot \vec{S}_1 \hat{n} \cdot \vec{S}_2 \hat{n} \cdot \vec{v}_1 \hat{n} \cdot \vec{v}_2 + 20 \vec{S}_1 \cdot \vec{S}_2 \hat{n} \cdot \vec{v}_1 \hat{n} \cdot \vec{v}_2 + \right. \right. \\ \left. \left. 8 \hat{n} \cdot \vec{S}_2 \hat{n} \cdot \vec{v}_2 \vec{S}_1 \cdot \vec{v}_1 - 8 \hat{n} \cdot \vec{S}_2 \hat{n} \cdot \vec{v}_2 \vec{S}_1 \cdot \vec{v}_2 + 8 \hat{n} \cdot \vec{S}_1 \hat{n} \cdot \vec{v}_2 \vec{S}_2 \cdot \vec{v}_1 - 8 \hat{n} \cdot \vec{S}_1 \hat{n} \cdot \vec{v}_2 \vec{S}_2 \cdot \vec{v}_2 + 8 \vec{v}_1 \cdot \vec{v}_2 \hat{n} \cdot \vec{S}_1 \hat{n} \cdot \vec{S}_2 - \right. \right. \\ \left. \left. 4 \vec{S}_1 \cdot \vec{S}_2 \vec{v}_1 \cdot \vec{v}_2 \right) + \frac{8 \hat{n} \cdot \vec{S}_2 \hat{n} \cdot \vec{S}_1 \hat{n} \cdot \vec{v}_2 + 8 \hat{n} \cdot \vec{S}_1 \hat{n} \cdot \vec{S}_2 \hat{n} \cdot \vec{v}_2 - 4 \vec{S}_1 \cdot \vec{S}_2 \hat{n} \cdot \vec{v}_2 - 4 \vec{S}_1 \cdot \vec{S}_2 \hat{n} \cdot \vec{v}_2}{r^4} \right\}$$

{DiagS1S2 [3, 6, 37],

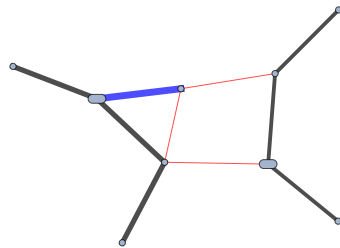

,  $-\frac{G^3 m_1 m_2 \hat{n} \times \vec{S}_1 \cdot \vec{v}_1 \hat{n} \times \vec{S}_2 \cdot \vec{v}_2}{r^5}$ }

{DiagS1S2 [3, 6, 38],

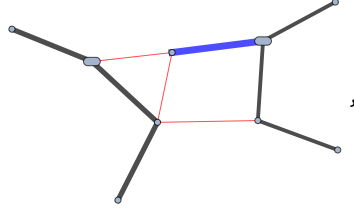

,

$$\frac{G^3 m_1 m_2 \left( -4 \hat{n} \times \vec{S}_1 \cdot \vec{v}_1 \hat{n} \times \vec{S}_2 \cdot \vec{v}_2 - \vec{S}_1 \cdot \vec{v}_2 \vec{S}_2 \cdot \vec{v}_1 + \vec{S}_1 \cdot \vec{S}_2 \vec{v}_1 \cdot \vec{v}_2 \right)}{r^5} \}$$

{DiagS1S2 [3, 6, 39],

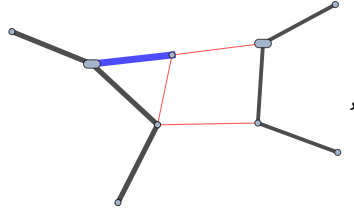

,

$$\frac{G^3 m_1 m_2 \left( -4 \hat{n} \times \vec{S}_1 \cdot \vec{v}_1 \hat{n} \times \vec{S}_2 \cdot \vec{v}_2 - \vec{S}_1 \cdot \vec{v}_2 \vec{S}_2 \cdot \vec{v}_1 + \vec{S}_1 \cdot \vec{S}_2 \vec{v}_1 \cdot \vec{v}_2 \right)}{r^5} \}$$

{DiagS1S2 [3, 6, 40],

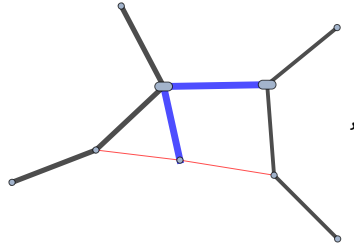

,

$$G^3 m_1 m_2 \left( \frac{2 \hat{n} \cdot \vec{a}_2 \hat{n} \cdot \vec{S}_1 \hat{n} \cdot \vec{S}_2 - 2 \vec{S}_1 \cdot \vec{S}_2 \hat{n} \cdot \vec{a}_2 + 2 \hat{n} \cdot \vec{S}_2 \hat{n} \cdot \vec{S}_1 \hat{n} \cdot \vec{v}_2 - 2 \vec{S}_1 \cdot \vec{S}_2 \hat{n} \cdot \vec{v}_2}{r^4} + \frac{1}{r^5} \right. \\ \left( \frac{15}{2} \hat{n} \times \vec{S}_1 \cdot \vec{v}_2 \hat{n} \times \vec{S}_2 \cdot \vec{v}_1 - 6 \hat{n} \times \vec{S}_1 \cdot \vec{v}_1 \hat{n} \times \vec{S}_2 \cdot \vec{v}_2 - 4 \hat{n} \times \vec{S}_1 \cdot \vec{v}_2 \hat{n} \times \vec{S}_2 \cdot \vec{v}_2 - 2 \hat{n} \cdot \vec{S}_1 \hat{n} \cdot \vec{S}_2 (\hat{n} \cdot \vec{v}_2)^2 + \right. \\ \left. 2 \vec{S}_1 \cdot \vec{S}_2 (\hat{n} \cdot \vec{v}_2)^2 + 2 \hat{n} \cdot \vec{S}_1 \hat{n} \cdot \vec{S}_2 \hat{n} \cdot \vec{v}_1 \hat{n} \cdot \vec{v}_2 - \frac{11}{2} \vec{S}_1 \cdot \vec{S}_2 \hat{n} \cdot \vec{v}_1 \hat{n} \cdot \vec{v}_2 - 2 \hat{n} \cdot \vec{S}_2 \hat{n} \cdot \vec{v}_2 \vec{S}_1 \cdot \vec{v}_1 - \right. \\ \left. 2 \hat{n} \cdot \vec{S}_2 \hat{n} \cdot \vec{v}_2 \vec{S}_1 \cdot \vec{v}_2 - \frac{5}{2} \hat{n} \cdot \vec{S}_1 \hat{n} \cdot \vec{v}_2 \vec{S}_2 \cdot \vec{v}_1 + 2 \hat{n} \cdot \vec{S}_1 \hat{n} \cdot \vec{v}_2 \vec{S}_2 \cdot \vec{v}_2 + 8 \hat{n} \cdot \vec{S}_2 \hat{n} \cdot \vec{v}_1 \vec{S}_1 \cdot \vec{v}_2 - \frac{19}{2} \vec{v}_1 \cdot \vec{v}_2 \hat{n} \cdot \vec{S}_1 \hat{n} \cdot \vec{S}_2 + \right. \\ \left. \left. 2 \vec{v}_2 \cdot \vec{v}_2 \hat{n} \cdot \vec{S}_1 \hat{n} \cdot \vec{S}_2 - 8 \vec{S}_1 \cdot \vec{v}_2 \vec{S}_2 \cdot \vec{v}_1 + 4 \vec{S}_1 \cdot \vec{v}_1 \vec{S}_2 \cdot \vec{v}_2 + \frac{11}{2} \vec{S}_1 \cdot \vec{S}_2 \vec{v}_1 \cdot \vec{v}_2 - 2 \vec{S}_1 \cdot \vec{S}_2 \vec{v}_2 \cdot \vec{v}_2 \right) \right) \}$$

{DiagS1S2 [3, 6, 41],

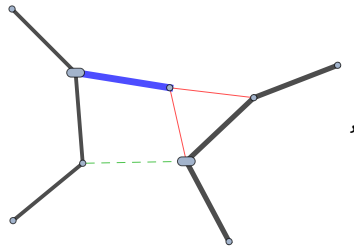

,

$$\frac{8 G^3 m_1 m_2 \hat{n} \times \vec{S}_1 \cdot \vec{v}_2 \hat{n} \times \vec{S}_2 \cdot \vec{v}_2}{r^5} \}$$

{DiagS1S2 [3, 6, 42],

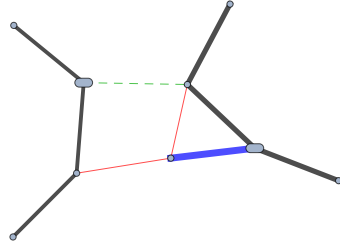

$$, \frac{G^3 m_1 m_2 \hat{n} \times \vec{S}_1 \cdot \vec{v}_1 \hat{n} \times \vec{S}_2 \cdot \vec{v}_1}{r^5} \}$$

{DiagS1S2 [3, 6, 43],

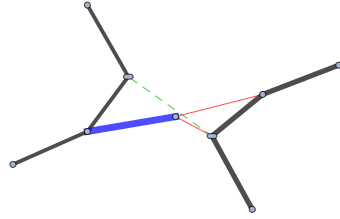

$$\frac{G^3 m_1 m_2 \left( 12 \hat{n} \cdot \vec{S}_1 \hat{n} \cdot \vec{S}_2 (\hat{n} \cdot \vec{v}_2)^2 - 4 \vec{S}_1 \cdot \vec{S}_2 (\hat{n} \cdot \vec{v}_2)^2 - 12 \vec{v}_2 \cdot \vec{v}_2 \hat{n} \cdot \vec{S}_1 \hat{n} \cdot \vec{S}_2 + 4 \vec{S}_1 \cdot \vec{S}_2 \vec{v}_2 \cdot \vec{v}_2 \right)}{r^5} \}$$

{DiagS1S2 [3, 6, 44],

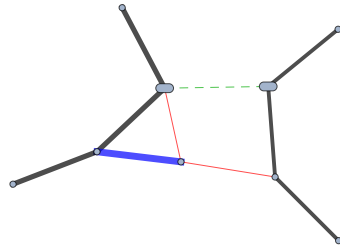

$$\frac{G^3 m_1 m_2 \left( -48 \hat{n} \cdot \vec{S}_1 \hat{n} \cdot \vec{S}_2 (\hat{n} \cdot \vec{v}_1)^2 + 16 \vec{S}_1 \cdot \vec{S}_2 (\hat{n} \cdot \vec{v}_1)^2 + 24 \vec{v}_1 \cdot \vec{v}_1 \hat{n} \cdot \vec{S}_1 \hat{n} \cdot \vec{S}_2 - 8 \vec{S}_1 \cdot \vec{S}_2 \vec{v}_1 \cdot \vec{v}_1 \right)}{r^5} \}$$

{DiagS1S2 [3, 6, 45],

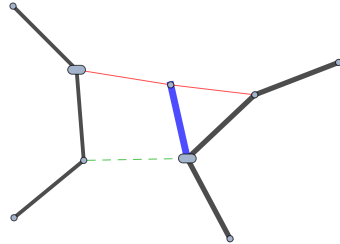

$$\frac{G^3 m_1 m_2 \left( 16 \hat{n} \times \vec{S}_1 \cdot \vec{v}_2 \hat{n} \times \vec{S}_2 \cdot \vec{v}_2 + 16 \vec{S}_1 \cdot \vec{S}_2 (\hat{n} \cdot \vec{v}_2)^2 - 16 \hat{n} \cdot \vec{S}_2 \hat{n} \cdot \vec{v}_2 \vec{S}_1 \cdot \vec{v}_2 + 16 \vec{S}_1 \cdot \vec{v}_2 \vec{S}_2 \cdot \vec{v}_2 - 16 \vec{S}_1 \cdot \vec{S}_2 \vec{v}_2 \cdot \vec{v}_2 \right)}{r^5} \}$$

{DiagS1S2 [3, 6, 46],

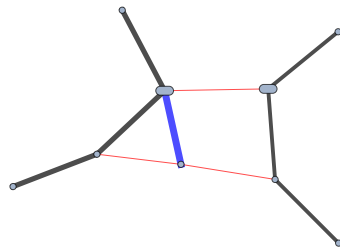

$$\frac{G^3 m_1 m_2 \left( -32 \hat{n} \times \vec{S}_1 \cdot \vec{v}_1 \hat{n} \times \vec{S}_2 \cdot \vec{v}_2 - 16 \vec{S}_1 \cdot \vec{S}_2 \hat{n} \cdot \vec{v}_1 \hat{n} \cdot \vec{v}_2 + 16 \hat{n} \cdot \vec{S}_2 \hat{n} \cdot \vec{v}_1 \vec{S}_1 \cdot \vec{v}_2 \right)}{r^5} \}$$



{DiagS1S2 [3, 6, 47],

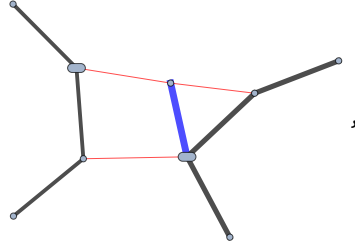

,

$$\frac{G^3 m_1 m_2 \left( -48 \hat{n} \times \vec{S}_1 \cdot \vec{v}_1 \hat{n} \times \vec{S}_2 \cdot \vec{v}_2 + 16 \vec{S}_1 \cdot \vec{S}_2 \hat{n} \cdot \vec{v}_1 \hat{n} \cdot \vec{v}_2 - 16 \hat{n} \cdot \vec{S}_2 \hat{n} \cdot \vec{v}_1 \vec{S}_1 \cdot \vec{v}_2 - 16 \vec{S}_1 \cdot \vec{v}_2 \vec{S}_2 \cdot \vec{v}_1 + 16 \vec{S}_1 \cdot \vec{S}_2 \vec{v}_1 \cdot \vec{v}_2 \right)}{r^5} \Bigg\}$$

{DiagS1S2 [3, 6, 48],

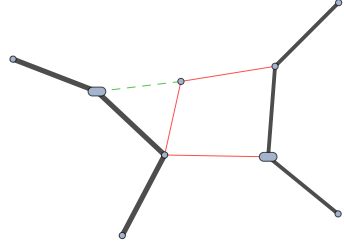

$$, \frac{G^3 m_1 m_2 \hat{n} \times \vec{S}_1 \cdot \vec{v}_1 \hat{n} \times \vec{S}_2 \cdot \vec{v}_2}{r^5} \Bigg\}$$

{DiagS1S2 [3, 6, 49],

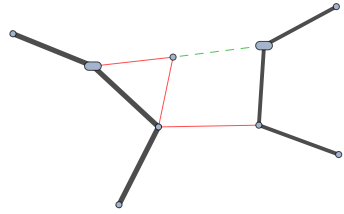

,

$$G^3 m_1 m_2 \left( \frac{\vec{S}_1 \cdot \vec{S}_2 \hat{n} \cdot \vec{a}_1 - \vec{S}_2 \cdot \vec{a}_1 \hat{n} \cdot \vec{S}_1 + \vec{S}_1 \cdot \vec{S}_2 \hat{n} \cdot \vec{v}_1 - \hat{n} \cdot \vec{S}_1 \vec{S}_2 \cdot \vec{v}_1}{r^4} + \frac{1}{r^5} \left( 4 \hat{n} \times \vec{S}_1 \cdot \vec{v}_1 \hat{n} \times \vec{S}_2 \cdot \vec{v}_1 + \vec{S}_1 \cdot \vec{S}_2 (\hat{n} \cdot \vec{v}_1)^2 - \right. \right. \\ \left. \left. \vec{S}_1 \cdot \vec{S}_2 \hat{n} \cdot \vec{v}_2 \hat{n} \cdot \vec{v}_1 - \hat{n} \cdot \vec{S}_1 \hat{n} \cdot \vec{v}_1 \vec{S}_2 \cdot \vec{v}_1 + \hat{n} \cdot \vec{S}_1 \hat{n} \cdot \vec{v}_2 \vec{S}_2 \cdot \vec{v}_1 + \vec{S}_1 \cdot \vec{v}_1 \vec{S}_2 \cdot \vec{v}_1 - \vec{S}_1 \cdot \vec{S}_2 \vec{v}_1 \cdot \vec{v}_1 \right) \right) \Bigg\}$$

{DiagS1S2 [3, 6, 50],

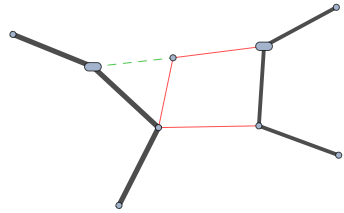

,

$$\frac{G^3 m_1 m_2 \left( 4 \hat{n} \times \vec{S}_1 \cdot \vec{v}_1 \hat{n} \times \vec{S}_2 \cdot \vec{v}_2 + \vec{S}_1 \cdot \vec{v}_2 \vec{S}_2 \cdot \vec{v}_1 - \vec{S}_1 \cdot \vec{S}_2 \vec{v}_1 \cdot \vec{v}_2 \right)}{r^5} \Bigg\}$$

{DiagS1S2 [3, 6, 51],

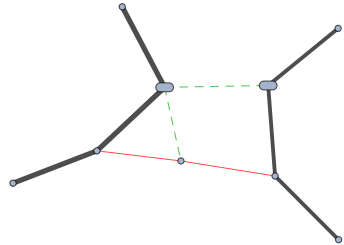

,  $G^3 m_1 m_2$

$$\left( \frac{1}{r^4} \left( -4 \hat{n} \cdot \vec{a}_1 \hat{n} \cdot \vec{S}_1 \hat{n} \cdot \vec{S}_2 - 4 \hat{n} \cdot \vec{a}_2 \hat{n} \cdot \vec{S}_1 \hat{n} \cdot \vec{S}_2 + 2 \vec{S}_1 \cdot \vec{S}_2 \hat{n} \cdot \vec{a}_1 + 2 \vec{S}_1 \cdot \vec{S}_2 \hat{n} \cdot \vec{a}_2 + 2 \vec{S}_2 \cdot \vec{a}_1 \hat{n} \cdot \vec{S}_1 + 2 \vec{S}_2 \cdot \vec{a}_2 \hat{n} \cdot \vec{S}_1 + \right. \right.$$

$$\begin{aligned}
& 4 \hat{n} \cdot \vec{S}_2 \hat{n} \cdot \vec{S}_1 \hat{n} \cdot \vec{v}_1 + 4 \hat{n} \cdot \vec{S}_2 \hat{n} \cdot \vec{S}_1 \hat{n} \cdot \vec{v}_2 - 2 \hat{n} \cdot \vec{S}_1 \vec{S}_2 \cdot \vec{v}_1 - 2 \hat{n} \cdot \vec{S}_1 \vec{S}_2 \cdot \vec{v}_2 - 2 \vec{S}_1 \cdot \vec{S}_2 \hat{n} \cdot \vec{v}_1 - 2 \vec{S}_1 \cdot \vec{S}_2 \hat{n} \cdot \vec{v}_2 \Big) + \\
& \frac{1}{r^5} \Big( -\hat{n} \times \vec{S}_1 \cdot \vec{v}_1 \hat{n} \times \vec{S}_2 \cdot \vec{v}_1 + 24 \hat{n} \cdot \vec{S}_1 \hat{n} \cdot \vec{S}_2 (\hat{n} \cdot \vec{v}_1)^2 - 10 \vec{S}_1 \cdot \vec{S}_2 (\hat{n} \cdot \vec{v}_1)^2 + 20 \hat{n} \cdot \vec{S}_1 \hat{n} \cdot \vec{S}_2 \hat{n} \cdot \vec{v}_2 \hat{n} \cdot \vec{v}_1 - \\
& 5 \vec{S}_1 \cdot \vec{S}_2 \hat{n} \cdot \vec{v}_2 \hat{n} \cdot \vec{v}_1 - 4 \hat{n} \cdot \vec{S}_2 \hat{n} \cdot \vec{v}_1 \vec{S}_1 \cdot \vec{v}_2 - 6 \hat{n} \cdot \vec{S}_1 \hat{n} \cdot \vec{v}_1 \vec{S}_2 \cdot \vec{v}_1 + \hat{n} \cdot \vec{S}_1 \hat{n} \cdot \vec{v}_1 \vec{S}_2 \cdot \vec{v}_2 - \\
& 4 \hat{n} \cdot \vec{S}_1 \hat{n} \cdot \vec{S}_2 (\hat{n} \cdot \vec{v}_2)^2 + 6 \vec{S}_1 \cdot \vec{S}_2 (\hat{n} \cdot \vec{v}_2)^2 - 4 \hat{n} \cdot \vec{S}_2 \hat{n} \cdot \vec{v}_2 \vec{S}_1 \cdot \vec{v}_2 - 4 \hat{n} \cdot \vec{S}_1 \hat{n} \cdot \vec{v}_2 \vec{S}_2 \cdot \vec{v}_1 + \\
& 2 \hat{n} \cdot \vec{S}_1 \hat{n} \cdot \vec{v}_2 \vec{S}_2 \cdot \vec{v}_2 - 8 \vec{v}_1 \cdot \vec{v}_2 \hat{n} \cdot \vec{S}_1 \hat{n} \cdot \vec{S}_2 - 5 \vec{v}_1 \cdot \vec{v}_2 \hat{n} \cdot \vec{S}_1 \hat{n} \cdot \vec{S}_2 + 4 \vec{v}_2 \cdot \vec{v}_2 \hat{n} \cdot \vec{S}_1 \hat{n} \cdot \vec{S}_2 + \\
& 2 \vec{S}_1 \cdot \vec{v}_2 \vec{S}_2 \cdot \vec{v}_1 + 2 \vec{S}_1 \cdot \vec{v}_2 \vec{S}_2 \cdot \vec{v}_2 + 4 \vec{S}_1 \cdot \vec{S}_2 \vec{v}_1 \cdot \vec{v}_1 - \vec{S}_1 \cdot \vec{S}_2 \vec{v}_1 \cdot \vec{v}_2 - 6 \vec{S}_1 \cdot \vec{S}_2 \vec{v}_2 \cdot \vec{v}_2 \Big) \Big\}
\end{aligned}$$

{DiagS1S2 [3, 6, 52],

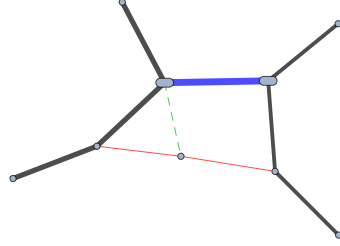

,  $\frac{1}{r^5}$

$$\begin{aligned}
& G^3 m_1 m_2 \left( \frac{1}{2} \hat{n} \times \vec{S}_1 \cdot \vec{v}_2 \hat{n} \times \vec{S}_2 \cdot \vec{v}_1 - 2 \hat{n} \times \vec{S}_1 \cdot \vec{v}_1 \hat{n} \times \vec{S}_2 \cdot \vec{v}_2 - \frac{1}{2} \vec{S}_1 \cdot \vec{S}_2 \hat{n} \cdot \vec{v}_1 \hat{n} \cdot \vec{v}_2 + \right. \\
& \left. \frac{1}{2} \hat{n} \cdot \vec{S}_1 \hat{n} \cdot \vec{v}_2 \vec{S}_2 \cdot \vec{v}_1 - \frac{1}{2} \vec{v}_1 \cdot \vec{v}_2 \hat{n} \cdot \vec{S}_1 \hat{n} \cdot \vec{S}_2 + \frac{1}{2} \vec{S}_1 \cdot \vec{S}_2 \vec{v}_1 \cdot \vec{v}_2 \right) \Big\}
\end{aligned}$$

{DiagS1S2 [3, 6, 53],

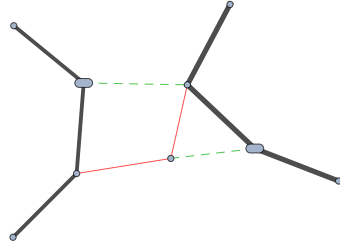

,  $-\frac{G^3 m_1 m_2 \hat{n} \times \vec{S}_1 \cdot \vec{v}_1 \hat{n} \times \vec{S}_2 \cdot \vec{v}_1}{r^5}$

{DiagS1S2 [3, 6, 54],

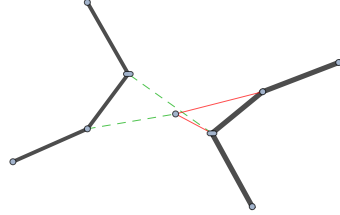

,

$$\begin{aligned}
& G^3 m_1 m_2 \left( \frac{1}{r^5} \left( 120 \hat{n} \cdot \vec{S}_1 \hat{n} \cdot \vec{S}_2 (\hat{n} \cdot \vec{v}_2)^2 - 24 \vec{S}_1 \cdot \vec{S}_2 (\hat{n} \cdot \vec{v}_2)^2 - 144 \hat{n} \cdot \vec{S}_1 \hat{n} \cdot \vec{S}_2 \hat{n} \cdot \vec{v}_1 \hat{n} \cdot \vec{v}_2 + \right. \right. \\
& 32 \vec{S}_1 \cdot \vec{S}_2 \hat{n} \cdot \vec{v}_1 \hat{n} \cdot \vec{v}_2 + 24 \hat{n} \cdot \vec{S}_2 \hat{n} \cdot \vec{v}_2 \vec{S}_1 \cdot \vec{v}_1 - 24 \hat{n} \cdot \vec{S}_2 \hat{n} \cdot \vec{v}_2 \vec{S}_1 \cdot \vec{v}_2 + \\
& 24 \hat{n} \cdot \vec{S}_1 \hat{n} \cdot \vec{v}_2 \vec{S}_2 \cdot \vec{v}_1 - 24 \hat{n} \cdot \vec{S}_1 \hat{n} \cdot \vec{v}_2 \vec{S}_2 \cdot \vec{v}_2 + 24 \vec{v}_1 \cdot \vec{v}_2 \hat{n} \cdot \vec{S}_1 \hat{n} \cdot \vec{S}_2 - 8 \vec{S}_1 \cdot \vec{S}_2 \vec{v}_1 \cdot \vec{v}_2 \Big) + \\
& \left. \frac{24 \hat{n} \cdot \vec{S}_2 \hat{n} \cdot \vec{S}_1 \hat{n} \cdot \vec{v}_2 + 24 \hat{n} \cdot \vec{S}_1 \hat{n} \cdot \vec{S}_2 \hat{n} \cdot \vec{v}_2 - 8 \vec{S}_1 \cdot \vec{S}_2 \hat{n} \cdot \vec{v}_2 - 8 \vec{S}_1 \cdot \vec{S}_2 \hat{n} \cdot \vec{v}_2}{r^4} \right) \Big\}
\end{aligned}$$

{DiagS1S2 [3, 6, 55],

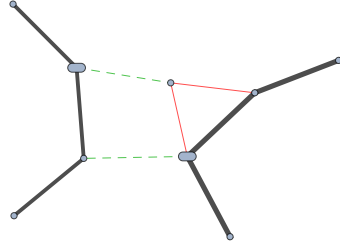

$$, - \frac{8 G^3 m_1 m_2 \hat{n} \times \vec{S}_1 \cdot \vec{v}_2 \hat{n} \times \vec{S}_2 \cdot \vec{v}_1}{r^5} \}$$

{DiagS1S2 [3, 6, 56],

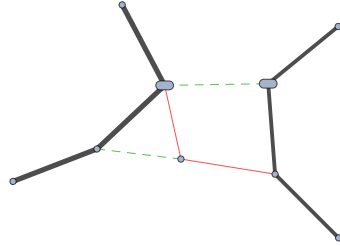

,

$$G^3 m_1 m_2 \left\{ \frac{1}{r^5} \left( 288 \hat{n} \cdot \vec{S}_1 \hat{n} \cdot \vec{S}_2 (\hat{n} \cdot \vec{v}_1)^2 - 64 \vec{S}_1 \cdot \vec{S}_2 (\hat{n} \cdot \vec{v}_1)^2 - 192 \hat{n} \cdot \vec{S}_1 \hat{n} \cdot \vec{S}_2 \hat{n} \cdot \vec{v}_2 \hat{n} \cdot \vec{v}_1 + \right. \right. \\ \left. 32 \vec{S}_1 \cdot \vec{S}_2 \hat{n} \cdot \vec{v}_2 \hat{n} \cdot \vec{v}_1 - 48 \hat{n} \cdot \vec{S}_2 \hat{n} \cdot \vec{v}_1 \vec{S}_1 \cdot \vec{v}_1 + 48 \hat{n} \cdot \vec{S}_2 \hat{n} \cdot \vec{v}_1 \vec{S}_1 \cdot \vec{v}_2 - 48 \hat{n} \cdot \vec{S}_1 \hat{n} \cdot \vec{v}_1 \vec{S}_2 \cdot \vec{v}_1 + \right. \\ \left. 48 \hat{n} \cdot \vec{S}_1 \hat{n} \cdot \vec{v}_1 \vec{S}_2 \cdot \vec{v}_2 - 24 \vec{v}_1 \cdot \vec{v}_1 \hat{n} \cdot \vec{S}_1 \hat{n} \cdot \vec{S}_2 - 24 \vec{v}_1 \cdot \vec{v}_2 \hat{n} \cdot \vec{S}_1 \hat{n} \cdot \vec{S}_2 + 8 \vec{S}_1 \cdot \vec{S}_2 \vec{v}_1 \cdot \vec{v}_1 + 8 \vec{S}_1 \cdot \vec{S}_2 \vec{v}_1 \cdot \vec{v}_2 \right) + \\ \left. \frac{-48 \hat{n} \cdot \vec{S}_2 \hat{n} \cdot \vec{S}_1 \hat{n} \cdot \vec{v}_1 - 48 \hat{n} \cdot \vec{S}_1 \hat{n} \cdot \vec{S}_2 \hat{n} \cdot \vec{v}_1 + 16 \vec{S}_1 \cdot \vec{S}_2 \hat{n} \cdot \vec{v}_1 + 16 \vec{S}_1 \cdot \vec{S}_2 \hat{n} \cdot \vec{v}_1}{r^4} \right\}$$

{DiagS1S2 [3, 6, 57],

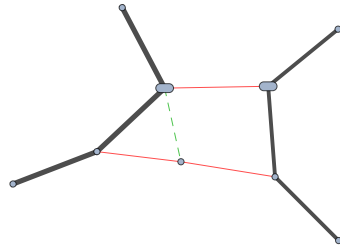

$$, \frac{4 G^3 m_1 m_2 \hat{n} \times \vec{S}_1 \cdot \vec{v}_1 \hat{n} \times \vec{S}_2 \cdot \vec{v}_2}{r^5} \}$$

{DiagS1S2 [3, 6, 58],

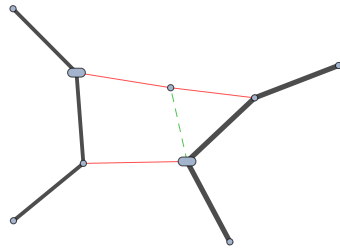

,

$$\frac{G^3 m_1 m_2 \left( 16 \hat{n} \times \vec{S}_1 \cdot \vec{v}_1 \hat{n} \times \vec{S}_2 \cdot \vec{v}_2 + 4 \vec{S}_1 \cdot \vec{v}_2 \vec{S}_2 \cdot \vec{v}_1 - 4 \vec{S}_1 \cdot \vec{S}_2 \vec{v}_1 \cdot \vec{v}_2 \right)}{r^5} \}$$

{DiagS1S2 [3, 6, 59],

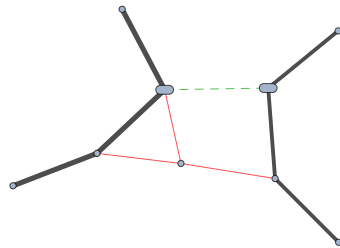

,

$$G^3 m_1 m_2 \left( \frac{1}{r^5} \left( 132 \hat{n} \cdot \vec{S}_1 \hat{n} \cdot \vec{S}_2 (\hat{n} \cdot \vec{v}_1)^2 - 28 \vec{S}_1 \cdot \vec{S}_2 (\hat{n} \cdot \vec{v}_1)^2 - 456 \hat{n} \cdot \vec{S}_1 \hat{n} \cdot \vec{S}_2 \hat{n} \cdot \vec{v}_2 \hat{n} \cdot \vec{v}_1 + 104 \vec{S}_1 \cdot \vec{S}_2 \hat{n} \cdot \vec{v}_2 \hat{n} \cdot \vec{v}_1 - \right. \right. \\ \left. 24 \hat{n} \cdot \vec{S}_2 \hat{n} \cdot \vec{v}_1 \vec{S}_1 \cdot \vec{v}_1 + 24 \hat{n} \cdot \vec{S}_2 \hat{n} \cdot \vec{v}_1 \vec{S}_1 \cdot \vec{v}_2 - 24 \hat{n} \cdot \vec{S}_1 \hat{n} \cdot \vec{v}_1 \vec{S}_2 \cdot \vec{v}_1 + 24 \hat{n} \cdot \vec{S}_1 \hat{n} \cdot \vec{v}_1 \vec{S}_2 \cdot \vec{v}_2 + 240 \hat{n} \cdot \vec{S}_1 \hat{n} \cdot \vec{S}_2 \right. \\ \left. (\hat{n} \cdot \vec{v}_2)^2 - 48 \vec{S}_1 \cdot \vec{S}_2 (\hat{n} \cdot \vec{v}_2)^2 + 48 \hat{n} \cdot \vec{S}_2 \hat{n} \cdot \vec{v}_2 \vec{S}_1 \cdot \vec{v}_1 - 48 \hat{n} \cdot \vec{S}_2 \hat{n} \cdot \vec{v}_2 \vec{S}_1 \cdot \vec{v}_2 + 48 \hat{n} \cdot \vec{S}_1 \hat{n} \cdot \vec{v}_2 \vec{S}_2 \cdot \vec{v}_1 - \right. \\ \left. 48 \hat{n} \cdot \vec{S}_1 \hat{n} \cdot \vec{v}_2 \vec{S}_2 \cdot \vec{v}_2 - 12 \vec{v}_1 \cdot \vec{v}_1 \hat{n} \cdot \vec{S}_1 \hat{n} \cdot \vec{S}_2 + 48 \vec{v}_1 \cdot \vec{v}_2 \hat{n} \cdot \vec{S}_1 \hat{n} \cdot \vec{S}_2 + 4 \vec{S}_1 \cdot \vec{S}_2 \vec{v}_1 \cdot \vec{v}_1 - 16 \vec{S}_1 \cdot \vec{S}_2 \vec{v}_1 \cdot \vec{v}_2 \right) + \\ \left. \frac{1}{r^4} \left( -24 \hat{n} \cdot \vec{S}_2 \hat{n} \cdot \vec{S}_1 \hat{n} \cdot \vec{v}_1 - 24 \hat{n} \cdot \vec{S}_1 \hat{n} \cdot \vec{S}_2 \hat{n} \cdot \vec{v}_1 + 8 \vec{S}_1 \cdot \vec{S}_2 \hat{n} \cdot \vec{v}_1 + 8 \vec{S}_1 \cdot \vec{S}_2 \hat{n} \cdot \vec{v}_1 + \right. \right. \\ \left. 48 \hat{n} \cdot \vec{S}_2 \hat{n} \cdot \vec{S}_1 \hat{n} \cdot \vec{v}_2 + 48 \hat{n} \cdot \vec{S}_1 \hat{n} \cdot \vec{S}_2 \hat{n} \cdot \vec{v}_2 - 16 \vec{S}_1 \cdot \vec{S}_2 \hat{n} \cdot \vec{v}_2 - 16 \vec{S}_1 \cdot \vec{S}_2 \hat{n} \cdot \vec{v}_2 \right) \Bigg) \Bigg\}$$

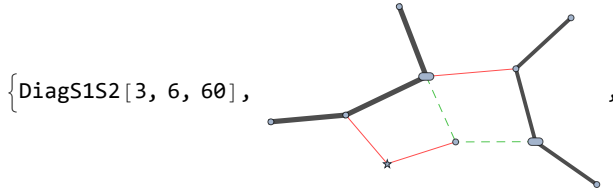

$$G^3 m_1 m_2 \left( \frac{1}{r^5} \left( 8 \hat{n} \times \vec{S}_1 \cdot \vec{v}_1 \hat{n} \times \vec{S}_2 \cdot \vec{v}_1 + 88 \hat{n} \cdot \vec{S}_1 \hat{n} \cdot \vec{S}_2 (\hat{n} \cdot \vec{v}_1)^2 - 14 \vec{S}_1 \cdot \vec{S}_2 (\hat{n} \cdot \vec{v}_1)^2 - 112 \hat{n} \cdot \vec{S}_1 \hat{n} \cdot \vec{S}_2 \hat{n} \cdot \vec{v}_2 \hat{n} \cdot \vec{v}_1 + \right. \right. \\ \left. 30 \vec{S}_1 \cdot \vec{S}_2 \hat{n} \cdot \vec{v}_2 \hat{n} \cdot \vec{v}_1 - 28 \hat{n} \cdot \vec{S}_2 \hat{n} \cdot \vec{v}_1 \vec{S}_1 \cdot \vec{v}_1 + 16 \hat{n} \cdot \vec{S}_2 \hat{n} \cdot \vec{v}_1 \vec{S}_1 \cdot \vec{v}_2 - 14 \hat{n} \cdot \vec{S}_1 \hat{n} \cdot \vec{v}_1 \vec{S}_2 \cdot \vec{v}_1 + \right. \\ \left. 16 \hat{n} \cdot \vec{S}_1 \hat{n} \cdot \vec{v}_1 \vec{S}_2 \cdot \vec{v}_2 + 20 \hat{n} \cdot \vec{S}_2 \hat{n} \cdot \vec{v}_2 \vec{S}_1 \cdot \vec{v}_1 - 10 \hat{n} \cdot \vec{S}_1 \hat{n} \cdot \vec{v}_2 \vec{S}_2 \cdot \vec{v}_1 + 16 \vec{v}_1 \cdot \vec{v}_2 \hat{n} \cdot \vec{S}_1 \hat{n} \cdot \vec{S}_2 + \right. \\ \left. 6 \vec{S}_1 \cdot \vec{v}_1 \vec{S}_2 \cdot \vec{v}_1 + 2 \vec{S}_1 \cdot \vec{v}_2 \vec{S}_2 \cdot \vec{v}_1 - 4 \vec{S}_1 \cdot \vec{v}_1 \vec{S}_2 \cdot \vec{v}_2 - 6 \vec{S}_1 \cdot \vec{S}_2 \vec{v}_1 \cdot \vec{v}_1 - 6 \vec{S}_1 \cdot \vec{S}_2 \vec{v}_1 \cdot \vec{v}_2 \right) + \\ \left. \frac{1}{r^4} \left( -16 \hat{n} \cdot \vec{S}_2 \hat{n} \cdot \vec{S}_1 \hat{n} \cdot \vec{v}_1 - 16 \hat{n} \cdot \vec{S}_1 \hat{n} \cdot \vec{S}_2 \hat{n} \cdot \vec{v}_1 + 6 \vec{S}_1 \cdot \vec{S}_2 \hat{n} \cdot \vec{v}_1 + 6 \vec{S}_1 \cdot \vec{S}_2 \hat{n} \cdot \vec{v}_1 + \right. \right. \\ \left. 4 \hat{n} \cdot \vec{S}_2 \vec{S}_1 \cdot \vec{v}_1 - 2 \hat{n} \cdot \vec{S}_1 \vec{S}_2 \cdot \vec{v}_1 + 4 \hat{n} \cdot \vec{S}_2 \vec{S}_1 \cdot \vec{v}_1 - 2 \hat{n} \cdot \vec{S}_1 \vec{S}_2 \cdot \vec{v}_1 \right) \Bigg) \Bigg\}$$

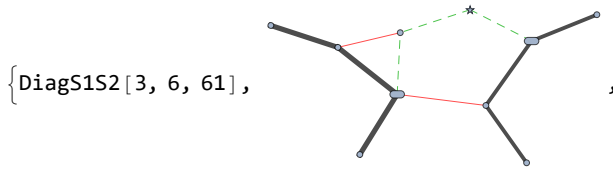

$$G^3 m_1 m_2 \left( \frac{1}{r^5} \left( 16 \hat{n} \cdot \vec{S}_1 \hat{n} \cdot \vec{S}_2 (\hat{n} \cdot \vec{v}_2)^2 - 112 \hat{n} \cdot \vec{S}_1 \hat{n} \cdot \vec{S}_2 \hat{n} \cdot \vec{v}_1 \hat{n} \cdot \vec{v}_2 + 16 \hat{n} \cdot \vec{S}_2 \hat{n} \cdot \vec{v}_2 \vec{S}_1 \cdot \vec{v}_1 - 4 \hat{n} \cdot \vec{S}_2 \hat{n} \cdot \vec{v}_2 \vec{S}_1 \cdot \vec{v}_2 + \right. \right. \\ \left. 16 \hat{n} \cdot \vec{S}_1 \hat{n} \cdot \vec{v}_2 \vec{S}_2 \cdot \vec{v}_1 - 4 \hat{n} \cdot \vec{S}_1 \hat{n} \cdot \vec{v}_2 \vec{S}_2 \cdot \vec{v}_2 + 20 \hat{n} \cdot \vec{S}_2 \hat{n} \cdot \vec{v}_1 \vec{S}_1 \cdot \vec{v}_2 + 20 \hat{n} \cdot \vec{S}_1 \hat{n} \cdot \vec{v}_1 \vec{S}_2 \cdot \vec{v}_2 + \right. \\ \left. 16 \vec{v}_1 \cdot \vec{v}_2 \hat{n} \cdot \vec{S}_1 \hat{n} \cdot \vec{S}_2 - 4 \vec{S}_1 \cdot \vec{v}_2 \vec{S}_2 \cdot \vec{v}_1 - 4 \vec{S}_1 \cdot \vec{v}_1 \vec{S}_2 \cdot \vec{v}_2 \right) + \frac{1}{r^4} \left( -20 \hat{n} \cdot \vec{S}_2 \hat{n} \cdot \vec{S}_1 \hat{n} \cdot \vec{v}_1 + 4 \hat{n} \cdot \vec{S}_2 \hat{n} \cdot \vec{S}_1 \hat{n} \cdot \vec{v}_2 + \right. \\ \left. 16 \hat{n} \cdot \vec{S}_1 \hat{n} \cdot \vec{S}_2 \hat{n} \cdot \vec{v}_2 - 4 \hat{n} \cdot \vec{S}_2 \vec{S}_1 \cdot \vec{v}_2 + 4 \hat{n} \cdot \vec{S}_1 \vec{S}_2 \cdot \vec{v}_1 + 4 \hat{n} \cdot \vec{S}_2 \vec{S}_1 \cdot \vec{v}_1 - 4 \hat{n} \cdot \vec{S}_1 \vec{S}_2 \cdot \vec{v}_2 \right) + \frac{4 \hat{n} \cdot \vec{S}_1 \hat{n} \cdot \vec{S}_2}{r^3} \Bigg) \Bigg\}$$

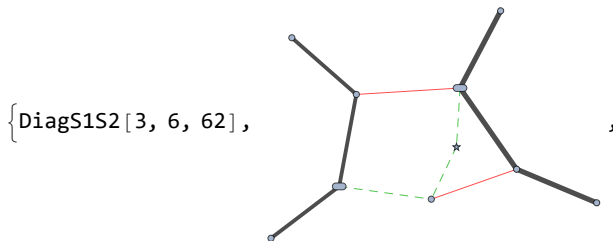

$$G^3 \left\{ \frac{24 \hat{n} \cdot \vec{S}_1 \hat{n} \cdot \vec{S}_2}{r^3} + \frac{1}{r^4} \left( -72 \hat{n} \cdot \vec{S}_2 \hat{n} \cdot \vec{S}_1 \hat{n} \cdot \vec{v}_1 - 48 \hat{n} \cdot \vec{S}_1 \hat{n} \cdot \vec{S}_2 \hat{n} \cdot \vec{v}_1 + \right. \right. \\ \left. \left. 2 \vec{S}_1 \cdot \vec{S}_2 \hat{n} \cdot \vec{v}_1 - 2 \vec{S}_1 \cdot \vec{S}_2 \hat{n} \cdot \vec{v}_1 + 24 \hat{n} \cdot \vec{S}_2 \hat{n} \cdot \vec{S}_1 \hat{n} \cdot \vec{v}_2 + 96 \hat{n} \cdot \vec{S}_1 \hat{n} \cdot \vec{S}_2 \hat{n} \cdot \vec{v}_2 + 12 \hat{n} \cdot \vec{S}_2 \vec{S}_1 \cdot \vec{v}_1 - \right. \right. \\ \left. \left. 24 \hat{n} \cdot \vec{S}_2 \vec{S}_1 \cdot \vec{v}_2 + 14 \hat{n} \cdot \vec{S}_1 \vec{S}_2 \cdot \vec{v}_1 + 12 \hat{n} \cdot \vec{S}_2 \vec{S}_1 \cdot \vec{v}_1 + 10 \hat{n} \cdot \vec{S}_1 \vec{S}_2 \cdot \vec{v}_1 - 24 \hat{n} \cdot \vec{S}_1 \vec{S}_2 \cdot \vec{v}_2 \right) + \frac{1}{r^5} \right. \\ \left. \left( 120 \hat{n} \cdot \vec{S}_1 \hat{n} \cdot \vec{S}_2 (\hat{n} \cdot \vec{v}_1)^2 + 6 \vec{S}_1 \cdot \vec{S}_2 (\hat{n} \cdot \vec{v}_1)^2 - 432 \hat{n} \cdot \vec{S}_1 \hat{n} \cdot \vec{S}_2 \hat{n} \cdot \vec{v}_2 \hat{n} \cdot \vec{v}_1 - 6 \hat{n} \cdot \vec{v}_2 \vec{S}_1 \cdot \vec{S}_2 \hat{n} \cdot \vec{v}_1 - \right. \right. \\ \left. \left. 36 \hat{n} \cdot \vec{S}_2 \vec{S}_1 \cdot \vec{v}_1 \hat{n} \cdot \vec{v}_1 + 72 \hat{n} \cdot \vec{S}_2 \vec{S}_1 \cdot \vec{v}_2 \hat{n} \cdot \vec{v}_1 - 42 \hat{n} \cdot \vec{S}_1 \vec{S}_2 \cdot \vec{v}_1 \hat{n} \cdot \vec{v}_1 + 72 \hat{n} \cdot \vec{S}_1 \vec{S}_2 \cdot \vec{v}_2 \hat{n} \cdot \vec{v}_1 + \right. \right. \\ \left. \left. 96 \hat{n} \cdot \vec{S}_1 \hat{n} \cdot \vec{S}_2 (\hat{n} \cdot \vec{v}_2)^2 + 8 \hat{n} \cdot \vec{S}_1 \cdot \vec{v}_1 \hat{n} \cdot \vec{S}_2 \cdot \vec{v}_1 + 60 \hat{n} \cdot \vec{S}_2 \hat{n} \cdot \vec{v}_2 \vec{S}_1 \cdot \vec{v}_1 - 24 \hat{n} \cdot \vec{S}_2 \hat{n} \cdot \vec{v}_2 \vec{S}_1 \cdot \vec{v}_2 + \right. \right. \\ \left. \left. 66 \hat{n} \cdot \vec{S}_1 \hat{n} \cdot \vec{v}_2 \vec{S}_2 \cdot \vec{v}_1 + 10 \vec{S}_1 \cdot \vec{v}_1 \vec{S}_2 \cdot \vec{v}_1 - 14 \vec{S}_1 \cdot \vec{v}_2 \vec{S}_2 \cdot \vec{v}_1 - 24 \hat{n} \cdot \vec{S}_1 \hat{n} \cdot \vec{v}_2 \vec{S}_2 \cdot \vec{v}_2 - 12 \vec{S}_1 \cdot \vec{v}_1 \vec{S}_2 \cdot \vec{v}_2 - \right. \right. \\ \left. \left. 16 \hat{n} \cdot \vec{S}_1 \hat{n} \cdot \vec{S}_2 \vec{v}_1 \cdot \vec{v}_1 - 2 \vec{S}_1 \cdot \vec{S}_2 \vec{v}_1 \cdot \vec{v}_1 + 48 \hat{n} \cdot \vec{S}_1 \hat{n} \cdot \vec{S}_2 \vec{v}_1 \cdot \vec{v}_2 + 2 \vec{S}_1 \cdot \vec{S}_2 \vec{v}_1 \cdot \vec{v}_2 \right) \right\} m_1 m_2 \}$$

{DiagS1S2 [3, 6, 63],

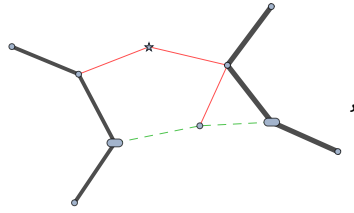

$$G^3 m_1 m_2 \left\{ \frac{1}{r^5} \left( 12 \hat{n} \cdot \vec{S}_1 \hat{n} \cdot \vec{S}_2 (\hat{n} \cdot \vec{v}_2)^2 - 4 \vec{S}_1 \cdot \vec{S}_2 (\hat{n} \cdot \vec{v}_2)^2 - 14 \hat{n} \cdot \vec{S}_1 \hat{n} \cdot \vec{S}_2 \hat{n} \cdot \vec{v}_1 \hat{n} \cdot \vec{v}_2 + 5 \vec{S}_1 \cdot \vec{S}_2 \hat{n} \cdot \vec{v}_1 \hat{n} \cdot \vec{v}_2 + \right. \right. \\ \left. \left. 2 \hat{n} \cdot \vec{S}_2 \hat{n} \cdot \vec{v}_2 \vec{S}_1 \cdot \vec{v}_1 - 2 \hat{n} \cdot \vec{S}_2 \hat{n} \cdot \vec{v}_2 \vec{S}_1 \cdot \vec{v}_2 + 2 \hat{n} \cdot \vec{S}_1 \hat{n} \cdot \vec{v}_2 \vec{S}_2 \cdot \vec{v}_1 - 2 \hat{n} \cdot \vec{S}_1 \hat{n} \cdot \vec{v}_2 \vec{S}_2 \cdot \vec{v}_2 + 2 \vec{v}_1 \cdot \vec{v}_2 \hat{n} \cdot \vec{S}_1 \hat{n} \cdot \vec{S}_2 - \right. \right. \\ \left. \left. \vec{S}_1 \cdot \vec{S}_2 \vec{v}_1 \cdot \vec{v}_2 \right) + \frac{2 \hat{n} \cdot \vec{S}_2 \hat{n} \cdot \vec{S}_1 \hat{n} \cdot \vec{v}_2 + 2 \hat{n} \cdot \vec{S}_1 \hat{n} \cdot \vec{S}_2 \hat{n} \cdot \vec{v}_2 - \vec{S}_1 \cdot \vec{S}_2 \hat{n} \cdot \vec{v}_2 - \vec{S}_1 \cdot \vec{S}_2 \hat{n} \cdot \vec{v}_2}{r^4} \right\}$$

{DiagS1S2 [3, 6, 64],

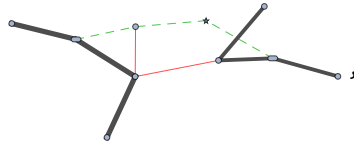

$$G^3 m_1 m_2 \left\{ \frac{1}{r^5} \left( 4 \hat{n} \cdot \vec{S}_1 \hat{n} \cdot \vec{S}_2 (\hat{n} \cdot \vec{v}_2)^2 - 28 \hat{n} \cdot \vec{S}_1 \hat{n} \cdot \vec{S}_2 \hat{n} \cdot \vec{v}_1 \hat{n} \cdot \vec{v}_2 + 4 \hat{n} \cdot \vec{S}_2 \hat{n} \cdot \vec{v}_2 \vec{S}_1 \cdot \vec{v}_1 - \hat{n} \cdot \vec{S}_2 \hat{n} \cdot \vec{v}_2 \vec{S}_1 \cdot \vec{v}_2 + \right. \right. \\ \left. \left. 4 \hat{n} \cdot \vec{S}_1 \hat{n} \cdot \vec{v}_2 \vec{S}_2 \cdot \vec{v}_1 - \hat{n} \cdot \vec{S}_1 \hat{n} \cdot \vec{v}_2 \vec{S}_2 \cdot \vec{v}_2 + 5 \hat{n} \cdot \vec{S}_2 \hat{n} \cdot \vec{v}_1 \vec{S}_1 \cdot \vec{v}_2 + 5 \hat{n} \cdot \vec{S}_1 \hat{n} \cdot \vec{v}_1 \vec{S}_2 \cdot \vec{v}_2 + \right. \right. \\ \left. \left. 4 \vec{v}_1 \cdot \vec{v}_2 \hat{n} \cdot \vec{S}_1 \hat{n} \cdot \vec{S}_2 - \vec{S}_1 \cdot \vec{v}_2 \vec{S}_2 \cdot \vec{v}_1 - \vec{S}_1 \cdot \vec{v}_1 \vec{S}_2 \cdot \vec{v}_2 \right) + \frac{1}{r^4} \left( -5 \hat{n} \cdot \vec{S}_2 \hat{n} \cdot \vec{S}_1 \hat{n} \cdot \vec{v}_1 + \hat{n} \cdot \vec{S}_2 \hat{n} \cdot \vec{S}_1 \hat{n} \cdot \vec{v}_2 + \right. \right. \\ \left. \left. 4 \hat{n} \cdot \vec{S}_1 \hat{n} \cdot \vec{S}_2 \hat{n} \cdot \vec{v}_2 - \hat{n} \cdot \vec{S}_2 \vec{S}_1 \cdot \vec{v}_2 + \hat{n} \cdot \vec{S}_1 \vec{S}_2 \cdot \vec{v}_1 + \hat{n} \cdot \vec{S}_2 \vec{S}_1 \cdot \vec{v}_1 - \hat{n} \cdot \vec{S}_1 \vec{S}_2 \cdot \vec{v}_2 \right) + \frac{\hat{n} \cdot \vec{S}_1 \hat{n} \cdot \vec{S}_2}{r^3} \right\}$$

{DiagS1S2 [3, 6, 65],

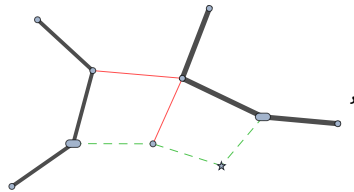

$$G^3 m_1 m_2 \left\{ \frac{1}{r^5} \left( 2 \hat{n} \times \vec{S}_1 \cdot \vec{v}_1 \hat{n} \times \vec{S}_2 \cdot \vec{v}_1 + 30 \hat{n} \cdot \vec{S}_1 \hat{n} \cdot \vec{S}_2 (\hat{n} \cdot \vec{v}_1)^2 + \frac{5}{2} \vec{S}_1 \cdot \vec{S}_2 (\hat{n} \cdot \vec{v}_1)^2 - 84 \hat{n} \cdot \vec{S}_1 \hat{n} \cdot \vec{S}_2 \hat{n} \cdot \vec{v}_2 \hat{n} \cdot \vec{v}_1 - \right. \right. \\ \left. \frac{5}{2} \vec{S}_1 \cdot \vec{S}_2 \hat{n} \cdot \vec{v}_2 \hat{n} \cdot \vec{v}_1 - 9 \hat{n} \cdot \vec{S}_2 \hat{n} \cdot \vec{v}_1 \vec{S}_1 \cdot \vec{v}_1 + 12 \hat{n} \cdot \vec{S}_2 \hat{n} \cdot \vec{v}_1 \vec{S}_1 \cdot \vec{v}_2 - \frac{23}{2} \hat{n} \cdot \vec{S}_1 \hat{n} \cdot \vec{v}_1 \vec{S}_2 \cdot \vec{v}_1 + \right. \\ \left. 12 \hat{n} \cdot \vec{S}_1 \hat{n} \cdot \vec{v}_1 \vec{S}_2 \cdot \vec{v}_2 + 15 \hat{n} \cdot \vec{S}_2 \hat{n} \cdot \vec{v}_2 \vec{S}_1 \cdot \vec{v}_1 + \frac{35}{2} \hat{n} \cdot \vec{S}_1 \hat{n} \cdot \vec{v}_2 \vec{S}_2 \cdot \vec{v}_1 - 4 \vec{v}_1 \cdot \vec{v}_1 \hat{n} \cdot \vec{S}_1 \hat{n} \cdot \vec{S}_2 + \right. \\ \left. 12 \vec{v}_1 \cdot \vec{v}_2 \hat{n} \cdot \vec{S}_1 \hat{n} \cdot \vec{S}_2 + \frac{5}{2} \vec{S}_1 \cdot \vec{v}_1 \vec{S}_2 \cdot \vec{v}_1 - \frac{7}{2} \vec{S}_1 \cdot \vec{v}_2 \vec{S}_2 \cdot \vec{v}_1 - 3 \vec{S}_1 \cdot \vec{v}_1 \vec{S}_2 \cdot \vec{v}_2 - \frac{1}{2} \vec{S}_1 \cdot \vec{S}_2 \vec{v}_1 \cdot \vec{v}_1 + \frac{1}{2} \vec{S}_1 \cdot \vec{S}_2 \vec{v}_1 \cdot \vec{v}_2 \right) + \\ \frac{1}{r^4} \left( -12 \hat{n} \cdot \vec{S}_2 \hat{n} \cdot \vec{S}_1 \hat{n} \cdot \vec{v}_1 - 18 \hat{n} \cdot \vec{S}_1 \hat{n} \cdot \vec{S}_2 \hat{n} \cdot \vec{v}_1 + \frac{1}{2} \vec{S}_1 \cdot \vec{S}_2 \hat{n} \cdot \vec{v}_1 - \frac{1}{2} \vec{S}_1 \cdot \vec{S}_2 \hat{n} \cdot \vec{v}_1 + 30 \hat{n} \cdot \vec{S}_1 \hat{n} \cdot \vec{S}_2 \hat{n} \cdot \vec{v}_2 + 3 \hat{n} \cdot \vec{S}_2 \right. \\ \left. \frac{1}{\vec{S}_1 \cdot \vec{v}_1} - 6 \hat{n} \cdot \vec{S}_2 \frac{1}{\vec{S}_1 \cdot \vec{v}_2} + \frac{7}{2} \hat{n} \cdot \vec{S}_1 \vec{S}_2 \cdot \vec{v}_1 + 3 \hat{n} \cdot \vec{S}_2 \vec{S}_1 \cdot \vec{v}_1 + \frac{5}{2} \hat{n} \cdot \vec{S}_1 \vec{S}_2 \cdot \vec{v}_1 - 6 \hat{n} \cdot \vec{S}_1 \vec{S}_2 \cdot \vec{v}_2 \right) + \frac{6 \hat{n} \cdot \vec{S}_1 \hat{n} \cdot \vec{S}_2}{r^3} \left. \right\}$$

{DiagS1S2 [3, 6, 66],

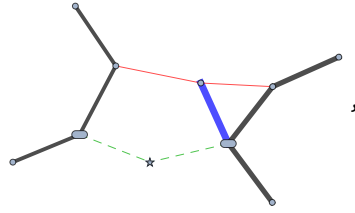

$$G^3 m_1 m_2 \left\{ \frac{1}{r^5} \left( -4 \hat{n} \times \vec{S}_1 \cdot \vec{v}_2 \hat{n} \times \vec{S}_2 \cdot \vec{v}_2 + 18 \hat{n} \cdot \vec{S}_1 \hat{n} \cdot \vec{S}_2 (\hat{n} \cdot \vec{v}_2)^2 - 4 \vec{S}_1 \cdot \vec{S}_2 (\hat{n} \cdot \vec{v}_2)^2 - 42 \hat{n} \cdot \vec{S}_1 \hat{n} \cdot \vec{S}_2 \hat{n} \cdot \vec{v}_1 \hat{n} \cdot \vec{v}_2 + \right. \right. \\ \left. 6 \hat{n} \cdot \vec{S}_2 \hat{n} \cdot \vec{v}_2 \vec{S}_1 \cdot \vec{v}_1 - 2 \hat{n} \cdot \vec{S}_2 \hat{n} \cdot \vec{v}_2 \vec{S}_1 \cdot \vec{v}_2 + 6 \hat{n} \cdot \vec{S}_1 \hat{n} \cdot \vec{v}_2 \vec{S}_2 \cdot \vec{v}_1 - 4 \hat{n} \cdot \vec{S}_1 \hat{n} \cdot \vec{v}_2 \vec{S}_2 \cdot \vec{v}_2 + 10 \hat{n} \cdot \vec{S}_1 \hat{n} \cdot \vec{v}_1 \vec{S}_2 \cdot \vec{v}_2 + \right. \\ \left. 6 \vec{v}_1 \cdot \vec{v}_2 \hat{n} \cdot \vec{S}_1 \hat{n} \cdot \vec{S}_2 - 2 \vec{v}_2 \cdot \vec{v}_2 \hat{n} \cdot \vec{S}_1 \hat{n} \cdot \vec{S}_2 - 2 \vec{S}_1 \cdot \vec{v}_1 \vec{S}_2 \cdot \vec{v}_2 - 2 \vec{S}_1 \cdot \vec{v}_2 \vec{S}_2 \cdot \vec{v}_2 + 4 \vec{S}_1 \cdot \vec{S}_2 \vec{v}_2 \cdot \vec{v}_2 \right) + \\ \frac{1}{r^4} \left( -20 \hat{n} \cdot \vec{S}_2 \hat{n} \cdot \vec{S}_1 \hat{n} \cdot \vec{v}_1 + 14 \hat{n} \cdot \vec{S}_2 \hat{n} \cdot \vec{S}_1 \hat{n} \cdot \vec{v}_2 + 6 \hat{n} \cdot \vec{S}_1 \hat{n} \cdot \vec{S}_2 \hat{n} \cdot \vec{v}_2 + 4 \hat{n} \cdot \vec{S}_1 \vec{S}_2 \cdot \vec{v}_1 - \right. \\ \left. 2 \hat{n} \cdot \vec{S}_1 \vec{S}_2 \cdot \vec{v}_2 + 4 \hat{n} \cdot \vec{S}_2 \vec{S}_1 \cdot \vec{v}_1 - 4 \hat{n} \cdot \vec{S}_2 \vec{S}_1 \cdot \vec{v}_2 - 2 \hat{n} \cdot \vec{S}_1 \vec{S}_2 \cdot \vec{v}_2 \right) + \frac{4 \hat{n} \cdot \vec{S}_1 \hat{n} \cdot \vec{S}_2}{r^3} \left. \right\}$$

{DiagS1S2 [3, 6, 67],

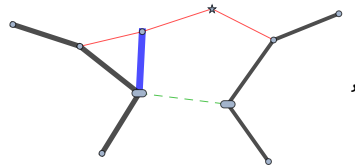

$$G^3 m_1 m_2 \left\{ \frac{1}{r^5} \left( -4 \hat{n} \times \vec{S}_1 \cdot \vec{v}_2 \hat{n} \times \vec{S}_2 \cdot \vec{v}_2 + 22 \hat{n} \cdot \vec{S}_1 \hat{n} \cdot \vec{S}_2 (\hat{n} \cdot \vec{v}_2)^2 - 8 \vec{S}_1 \cdot \vec{S}_2 (\hat{n} \cdot \vec{v}_2)^2 - \frac{98}{3} \hat{n} \cdot \vec{S}_1 \hat{n} \cdot \vec{S}_2 \hat{n} \cdot \vec{v}_1 \hat{n} \cdot \vec{v}_2 + \right. \right. \\ \frac{20}{3} \vec{S}_1 \cdot \vec{S}_2 \hat{n} \cdot \vec{v}_1 \hat{n} \cdot \vec{v}_2 + \frac{14}{3} \hat{n} \cdot \vec{S}_2 \hat{n} \cdot \vec{v}_2 \vec{S}_1 \cdot \vec{v}_1 - 6 \hat{n} \cdot \vec{S}_2 \hat{n} \cdot \vec{v}_2 \vec{S}_1 \cdot \vec{v}_2 + \frac{14}{3} \hat{n} \cdot \vec{S}_1 \hat{n} \cdot \vec{v}_2 \vec{S}_2 \cdot \vec{v}_1 + \\ \frac{20}{3} \hat{n} \cdot \vec{S}_2 \hat{n} \cdot \vec{v}_1 \vec{S}_1 \cdot \vec{v}_2 - \frac{10}{3} \hat{n} \cdot \vec{S}_1 \hat{n} \cdot \vec{v}_1 \vec{S}_2 \cdot \vec{v}_2 + \frac{14}{3} \vec{v}_1 \cdot \vec{v}_2 \hat{n} \cdot \vec{S}_1 \hat{n} \cdot \vec{S}_2 - 2 \vec{v}_2 \cdot \vec{v}_2 \hat{n} \cdot \vec{S}_1 \hat{n} \cdot \vec{S}_2 - \\ \frac{4}{3} \vec{S}_1 \cdot \vec{v}_2 \vec{S}_2 \cdot \vec{v}_1 + \frac{2}{3} \vec{S}_1 \cdot \vec{v}_1 \vec{S}_2 \cdot \vec{v}_2 - 2 \vec{S}_1 \cdot \vec{v}_2 \vec{S}_2 \cdot \vec{v}_2 - \frac{4}{3} \vec{S}_1 \cdot \vec{S}_2 \vec{v}_1 \cdot \vec{v}_2 + 4 \vec{S}_1 \cdot \vec{S}_2 \vec{v}_2 \cdot \vec{v}_2 \left. \right) + \\ \frac{1}{r^4} \left( \frac{14}{3} \hat{n} \cdot \vec{S}_2 \hat{n} \cdot \vec{S}_1 \hat{n} \cdot \vec{v}_2 + \frac{14}{3} \hat{n} \cdot \vec{S}_1 \hat{n} \cdot \vec{S}_2 \hat{n} \cdot \vec{v}_2 - \frac{4}{3} \vec{S}_1 \cdot \vec{S}_2 \hat{n} \cdot \vec{v}_2 - \frac{4}{3} \vec{S}_1 \cdot \vec{S}_2 \hat{n} \cdot \vec{v}_2 - \right. \\ \left. \frac{4}{3} \hat{n} \cdot \vec{S}_2 \vec{S}_1 \cdot \vec{v}_2 + \frac{2}{3} \hat{n} \cdot \vec{S}_1 \vec{S}_2 \cdot \vec{v}_2 - \frac{4}{3} \hat{n} \cdot \vec{S}_2 \vec{S}_1 \cdot \vec{v}_2 + \frac{2}{3} \hat{n} \cdot \vec{S}_1 \vec{S}_2 \cdot \vec{v}_2 \right) \left. \right\}$$

{DiagS1S2 [3, 6, 68],

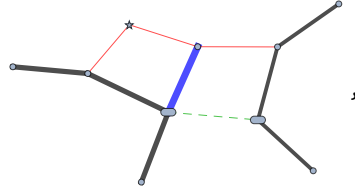

$$G^3 m_1 m_2 \left( \frac{1}{r^5} \left( -3 \hat{n} \cdot \vec{S}_1 \cdot \vec{v}_1 \hat{n} \cdot \vec{S}_2 \cdot \vec{v}_1 + \frac{64}{3} \hat{n} \cdot \vec{S}_1 \hat{n} \cdot \vec{S}_2 (\hat{n} \cdot \vec{v}_1)^2 - \frac{28}{3} \vec{S}_1 \cdot \vec{S}_2 (\hat{n} \cdot \vec{v}_1)^2 - \frac{161}{6} \hat{n} \cdot \vec{S}_1 \hat{n} \cdot \vec{S}_2 \hat{n} \cdot \vec{v}_2 \hat{n} \cdot \vec{v}_1 + \right. \right. \\ \left. \frac{25}{3} \vec{S}_1 \cdot \vec{S}_2 \hat{n} \cdot \vec{v}_2 \hat{n} \cdot \vec{v}_1 - \frac{55}{6} \hat{n} \cdot \vec{S}_2 \hat{n} \cdot \vec{v}_1 \vec{S}_1 \cdot \vec{v}_1 + \frac{23}{6} \hat{n} \cdot \vec{S}_2 \hat{n} \cdot \vec{v}_1 \vec{S}_1 \cdot \vec{v}_2 + \frac{11}{6} \hat{n} \cdot \vec{S}_1 \hat{n} \cdot \vec{v}_1 \vec{S}_2 \cdot \vec{v}_1 + \right. \\ \left. \frac{23}{6} \hat{n} \cdot \vec{S}_1 \hat{n} \cdot \vec{v}_1 \vec{S}_2 \cdot \vec{v}_2 + \frac{25}{3} \hat{n} \cdot \vec{S}_2 \hat{n} \cdot \vec{v}_2 \vec{S}_1 \cdot \vec{v}_1 - \frac{25}{6} \hat{n} \cdot \vec{S}_1 \hat{n} \cdot \vec{v}_2 \vec{S}_2 \cdot \vec{v}_1 - \frac{11}{6} \vec{v}_1 \cdot \vec{v}_1 \hat{n} \cdot \vec{S}_1 \hat{n} \cdot \vec{S}_2 + \frac{23}{6} \vec{v}_1 \cdot \vec{v}_2 \right. \\ \left. \hat{n} \cdot \vec{S}_1 \hat{n} \cdot \vec{S}_2 - \frac{7}{6} \vec{S}_1 \cdot \vec{v}_1 \vec{S}_2 \cdot \vec{v}_1 + \frac{5}{6} \vec{S}_1 \cdot \vec{v}_2 \vec{S}_2 \cdot \vec{v}_1 - \frac{5}{3} \vec{S}_1 \cdot \vec{v}_1 \vec{S}_2 \cdot \vec{v}_2 + \frac{11}{3} \vec{S}_1 \cdot \vec{S}_2 \vec{v}_1 \cdot \vec{v}_1 - \frac{5}{3} \vec{S}_1 \cdot \vec{S}_2 \vec{v}_1 \cdot \vec{v}_2 \right) + \\ \left. \frac{1}{r^4} \left( -\frac{23}{6} \hat{n} \cdot \vec{S}_2 \hat{n} \cdot \vec{S}_1 \hat{n} \cdot \vec{v}_1 - \frac{23}{6} \hat{n} \cdot \vec{S}_1 \hat{n} \cdot \vec{S}_2 \hat{n} \cdot \vec{v}_1 + \frac{5}{3} \vec{S}_1 \cdot \vec{S}_2 \hat{n} \cdot \vec{v}_1 + \frac{5}{3} \vec{S}_1 \cdot \vec{S}_2 \hat{n} \cdot \vec{v}_1 + \right. \right. \\ \left. \left. \frac{5}{3} \hat{n} \cdot \vec{S}_2 \vec{S}_1 \cdot \vec{v}_1 - \frac{5}{6} \hat{n} \cdot \vec{S}_1 \vec{S}_2 \cdot \vec{v}_1 + \frac{5}{3} \hat{n} \cdot \vec{S}_2 \vec{S}_1 \cdot \vec{v}_1 - \frac{5}{6} \hat{n} \cdot \vec{S}_1 \vec{S}_2 \cdot \vec{v}_1 \right) \right) \Bigg\}$$

{DiagS1S2 [3, 6, 69],

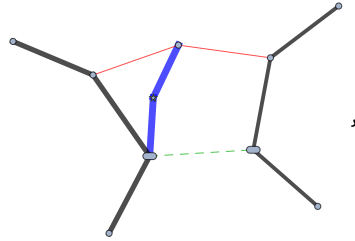

$$G^3 \left( \frac{1}{r^4} \left( \frac{11}{2} \hat{n} \cdot \vec{S}_2 \hat{n} \cdot \vec{S}_1 \hat{n} \cdot \vec{v}_1 + \frac{11}{2} \hat{n} \cdot \vec{S}_1 \hat{n} \cdot \vec{S}_2 \hat{n} \cdot \vec{v}_1 - \vec{S}_1 \cdot \vec{S}_2 \hat{n} \cdot \vec{v}_1 - \vec{S}_1 \cdot \vec{S}_2 \hat{n} \cdot \vec{v}_1 - \frac{14}{3} \hat{n} \cdot \vec{S}_2 \hat{n} \cdot \vec{S}_1 \hat{n} \cdot \vec{v}_2 - \right. \right. \\ \left. \frac{14}{3} \hat{n} \cdot \vec{S}_1 \hat{n} \cdot \vec{S}_2 \hat{n} \cdot \vec{v}_2 + \frac{4}{3} \hat{n} \cdot \vec{v}_2 \vec{S}_1 \cdot \vec{S}_2 - \hat{n} \cdot \vec{S}_2 \vec{S}_1 \cdot \vec{v}_1 + \frac{4}{3} \hat{n} \cdot \vec{S}_2 \vec{S}_1 \cdot \vec{v}_2 + \frac{1}{2} \hat{n} \cdot \vec{S}_1 \vec{S}_2 \cdot \vec{v}_1 - \right. \\ \left. \frac{2}{3} \hat{n} \cdot \vec{S}_1 \vec{S}_2 \cdot \vec{v}_2 + \frac{4}{3} \hat{n} \cdot \vec{v}_2 \vec{S}_1 \cdot \vec{S}_2 - \hat{n} \cdot \vec{S}_2 \vec{S}_1 \cdot \vec{v}_1 + \frac{4}{3} \hat{n} \cdot \vec{S}_2 \vec{S}_1 \cdot \vec{v}_2 + \frac{1}{2} \hat{n} \cdot \vec{S}_1 \vec{S}_2 \cdot \vec{v}_1 - \frac{2}{3} \hat{n} \cdot \vec{S}_1 \vec{S}_2 \cdot \vec{v}_2 \right) + \frac{1}{r^5} \\ \left( -23 \hat{n} \cdot \vec{S}_1 \hat{n} \cdot \vec{S}_2 (\hat{n} \cdot \vec{v}_1)^2 + 6 \vec{S}_1 \cdot \vec{S}_2 (\hat{n} \cdot \vec{v}_1)^2 + \frac{271}{6} \hat{n} \cdot \vec{S}_1 \hat{n} \cdot \vec{S}_2 \hat{n} \cdot \vec{v}_2 \hat{n} \cdot \vec{v}_1 - \frac{41}{3} \hat{n} \cdot \vec{v}_2 \vec{S}_1 \cdot \vec{S}_2 \hat{n} \cdot \vec{v}_1 + \right. \\ \left. \frac{7}{2} \hat{n} \cdot \vec{S}_2 \vec{S}_1 \cdot \vec{v}_1 \hat{n} \cdot \vec{v}_1 - \frac{25}{6} \hat{n} \cdot \vec{S}_2 \vec{S}_1 \cdot \vec{v}_2 \hat{n} \cdot \vec{v}_1 + \frac{7}{2} \hat{n} \cdot \vec{S}_1 \vec{S}_2 \cdot \vec{v}_1 \hat{n} \cdot \vec{v}_1 - \frac{19}{6} \hat{n} \cdot \vec{S}_1 \vec{S}_2 \cdot \vec{v}_2 \hat{n} \cdot \vec{v}_1 - \right. \\ \left. 22 \hat{n} \cdot \vec{S}_1 \hat{n} \cdot \vec{S}_2 (\hat{n} \cdot \vec{v}_2)^2 + 3 \hat{n} \cdot \vec{S}_1 \cdot \vec{v}_1 \hat{n} \cdot \vec{S}_2 \cdot \vec{v}_1 - 3 \hat{n} \cdot \vec{S}_1 \cdot \vec{v}_2 \hat{n} \cdot \vec{S}_2 \cdot \vec{v}_1 - 3 \hat{n} \cdot \vec{S}_1 \cdot \vec{v}_1 \hat{n} \cdot \vec{S}_2 \cdot \vec{v}_2 + \right. \\ \left. 4 \hat{n} \cdot \vec{S}_1 \cdot \vec{v}_2 \hat{n} \cdot \vec{S}_2 \cdot \vec{v}_2 + 8 (\hat{n} \cdot \vec{v}_2)^2 \vec{S}_1 \cdot \vec{S}_2 - \frac{17}{3} \hat{n} \cdot \vec{S}_2 \hat{n} \cdot \vec{v}_2 \vec{S}_1 \cdot \vec{v}_1 + 6 \hat{n} \cdot \vec{S}_2 \hat{n} \cdot \vec{v}_2 \vec{S}_1 \cdot \vec{v}_2 - \frac{7}{6} \hat{n} \cdot \vec{S}_1 \hat{n} \cdot \vec{v}_2 \vec{S}_2 \cdot \vec{v}_1 + \right. \\ \left. \frac{3}{2} \vec{S}_1 \cdot \vec{v}_1 \vec{S}_2 \cdot \vec{v}_1 - \frac{7}{6} \vec{S}_1 \cdot \vec{v}_2 \vec{S}_2 \cdot \vec{v}_1 - \frac{5}{3} \vec{S}_1 \cdot \vec{v}_1 \vec{S}_2 \cdot \vec{v}_2 + 2 \vec{S}_1 \cdot \vec{v}_2 \vec{S}_2 \cdot \vec{v}_2 + \frac{7}{2} \hat{n} \cdot \vec{S}_1 \hat{n} \cdot \vec{S}_2 \vec{v}_1 \cdot \vec{v}_1 - \right. \\ \left. 3 \vec{S}_1 \cdot \vec{S}_2 \vec{v}_1 \cdot \vec{v}_1 - \frac{13}{6} \hat{n} \cdot \vec{S}_1 \hat{n} \cdot \vec{S}_2 \vec{v}_1 \cdot \vec{v}_2 + \frac{19}{3} \vec{S}_1 \cdot \vec{S}_2 \vec{v}_1 \cdot \vec{v}_2 + 2 \hat{n} \cdot \vec{S}_1 \hat{n} \cdot \vec{S}_2 \vec{v}_2 \cdot \vec{v}_2 - 4 \vec{S}_1 \cdot \vec{S}_2 \vec{v}_2 \cdot \vec{v}_2 \right) \Bigg\} m_1 m_2 \Bigg\}$$

{DiagS1S2 [3, 6, 70],

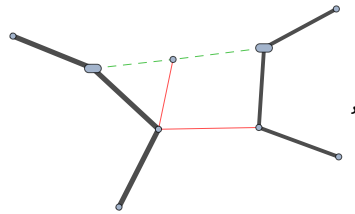

$$G^3 m_1 m_2 \left( \frac{1}{r^4} \left( -2 \vec{S}_1 \cdot \vec{a}_2 \hat{n} \cdot \vec{S}_2 - 8 \vec{S}_1 \cdot \vec{S}_2 \hat{n} \cdot \vec{a}_1 + 2 \vec{S}_1 \cdot \vec{S}_2 \hat{n} \cdot \vec{a}_2 + 8 \vec{S}_2 \cdot \vec{a}_1 \hat{n} \cdot \vec{S}_1 - 8 \vec{S}_1 \cdot \vec{S}_2 \hat{n} \cdot \vec{v}_1 + 2 \vec{S}_1 \cdot \vec{S}_2 \hat{n} \cdot \vec{v}_2 - \right. \right. \\ \left. \left. 2 \hat{n} \cdot \vec{S}_2 \vec{S}_1 \cdot \vec{v}_2 + 8 \hat{n} \cdot \vec{S}_1 \vec{S}_2 \cdot \vec{v}_1 \right) + \frac{1}{r^5} \left( -14 \hat{n} \times \vec{S}_1 \cdot \vec{v}_1 \hat{n} \times \vec{S}_2 \cdot \vec{v}_1 - 6 \hat{n} \times \vec{S}_1 \cdot \vec{v}_2 \hat{n} \times \vec{S}_2 \cdot \vec{v}_2 + 10 \vec{S}_1 \cdot \vec{S}_2 (\hat{n} \cdot \vec{v}_1)^2 - \right. \right. \\ \left. \left. 10 \hat{n} \cdot \vec{S}_1 \hat{n} \cdot \vec{v}_1 \vec{S}_2 \cdot \vec{v}_1 + 2 \vec{S}_1 \cdot \vec{S}_2 (\hat{n} \cdot \vec{v}_2)^2 - 2 \hat{n} \cdot \vec{S}_2 \hat{n} \cdot \vec{v}_2 \vec{S}_1 \cdot \vec{v}_2 - 18 \vec{v}_1 \cdot \vec{v}_1 \hat{n} \cdot \vec{S}_1 \hat{n} \cdot \vec{S}_2 + \right. \right. \\ \left. \left. 6 \vec{v}_2 \cdot \vec{v}_2 \hat{n} \cdot \vec{S}_1 \hat{n} \cdot \vec{S}_2 - \vec{S}_1 \cdot \vec{v}_1 \vec{S}_2 \cdot \vec{v}_1 - \vec{S}_1 \cdot \vec{v}_2 \vec{S}_2 \cdot \vec{v}_2 + 10 \vec{S}_1 \cdot \vec{S}_2 \vec{v}_1 \cdot \vec{v}_1 - 2 \vec{S}_1 \cdot \vec{S}_2 \vec{v}_2 \cdot \vec{v}_2 \right) \right) \Bigg\}$$

{DiagS1S2 [3, 6, 71],

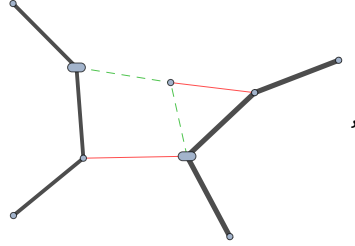

$$G^3 m_1 m_2 \left( \frac{-8 \vec{S}_1 \cdot \vec{a}_2 \hat{n} \cdot \vec{S}_2 + 8 \vec{S}_1 \cdot \vec{S}_2 \hat{n} \cdot \vec{a}_2 + 8 \vec{S}_1 \cdot \vec{S}_2 \hat{n} \cdot \vec{v}_2 - 8 \hat{n} \cdot \vec{S}_2 \vec{S}_1 \cdot \vec{v}_2}{r^4} + \frac{1}{r^5} \right. \\ \left( -24 \hat{n} \times \vec{S}_1 \cdot \vec{v}_2 \hat{n} \times \vec{S}_2 \cdot \vec{v}_2 + 8 \vec{S}_1 \cdot \vec{S}_2 (\hat{n} \cdot \vec{v}_2)^2 + 16 \vec{S}_1 \cdot \vec{S}_2 \hat{n} \cdot \vec{v}_1 \hat{n} \cdot \vec{v}_2 - 8 \hat{n} \cdot \vec{S}_2 \hat{n} \cdot \vec{v}_2 \vec{S}_1 \cdot \vec{v}_2 - 16 \hat{n} \cdot \vec{S}_1 \hat{n} \cdot \vec{v}_2 \vec{S}_2 \cdot \vec{v}_1 + \right. \\ \left. 24 \vec{v}_1 \cdot \vec{v}_1 \hat{n} \cdot \vec{S}_1 \hat{n} \cdot \vec{S}_2 + 24 \vec{v}_2 \cdot \vec{v}_2 \hat{n} \cdot \vec{S}_1 \hat{n} \cdot \vec{S}_2 - 4 \vec{S}_1 \cdot \vec{v}_2 \vec{S}_2 \cdot \vec{v}_2 - 12 \vec{S}_1 \cdot \vec{S}_2 \vec{v}_1 \cdot \vec{v}_1 - 8 \vec{S}_1 \cdot \vec{S}_2 \vec{v}_2 \cdot \vec{v}_2 \right) \Bigg\}$$

{DiagS1S2 [3, 6, 72],

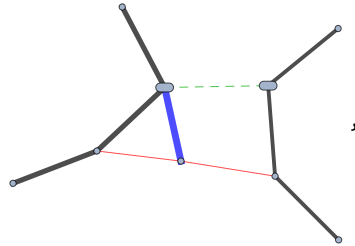

$$G^3 m_1 m_2 \left( \frac{1}{r^5} \left( 6 \hat{n} \times \vec{S}_1 \cdot \vec{v}_1 \hat{n} \times \vec{S}_2 \cdot \vec{v}_1 + 8 \hat{n} \times \vec{S}_1 \cdot \vec{v}_1 \hat{n} \times \vec{S}_2 \cdot \vec{v}_2 - 4 \hat{n} \times \vec{S}_1 \cdot \vec{v}_2 \hat{n} \times \vec{S}_2 \cdot \vec{v}_2 - 6 \hat{n} \cdot \vec{S}_1 \hat{n} \cdot \vec{S}_2 (\hat{n} \cdot \vec{v}_1)^2 + \right. \right. \\ \left. \left. 7 \vec{S}_1 \cdot \vec{S}_2 (\hat{n} \cdot \vec{v}_1)^2 + 32 \hat{n} \cdot \vec{S}_1 \hat{n} \cdot \vec{S}_2 \hat{n} \cdot \vec{v}_2 \hat{n} \cdot \vec{v}_1 - 8 \vec{S}_1 \cdot \vec{S}_2 \hat{n} \cdot \vec{v}_2 \hat{n} \cdot \vec{v}_1 - 12 \hat{n} \cdot \vec{S}_2 \hat{n} \cdot \vec{v}_1 \vec{S}_1 \cdot \vec{v}_1 + \right. \right. \\ \left. \left. 8 \hat{n} \cdot \vec{S}_2 \hat{n} \cdot \vec{v}_1 \vec{S}_1 \cdot \vec{v}_2 + 11 \hat{n} \cdot \vec{S}_1 \hat{n} \cdot \vec{v}_1 \vec{S}_2 \cdot \vec{v}_1 - 8 \hat{n} \cdot \vec{S}_1 \hat{n} \cdot \vec{v}_1 \vec{S}_2 \cdot \vec{v}_2 - 4 \vec{S}_1 \cdot \vec{S}_2 (\hat{n} \cdot \vec{v}_2)^2 + 4 \hat{n} \cdot \vec{S}_2 \hat{n} \cdot \vec{v}_2 \vec{S}_1 \cdot \vec{v}_2 - \right. \right. \\ \left. \left. 8 \hat{n} \cdot \vec{S}_1 \hat{n} \cdot \vec{v}_2 \vec{S}_2 \cdot \vec{v}_1 + 17 \vec{v}_1 \cdot \vec{v}_1 \hat{n} \cdot \vec{S}_1 \hat{n} \cdot \vec{S}_2 - 20 \vec{v}_1 \cdot \vec{v}_2 \hat{n} \cdot \vec{S}_1 \hat{n} \cdot \vec{S}_2 + 12 \vec{v}_2 \cdot \vec{v}_2 \hat{n} \cdot \vec{S}_1 \hat{n} \cdot \vec{S}_2 - 4 \vec{S}_1 \cdot \vec{v}_2 \vec{S}_2 \cdot \vec{v}_2 - \right. \right. \\ \left. \left. 5 \vec{S}_1 \cdot \vec{S}_2 \vec{v}_1 \cdot \vec{v}_1 + 12 \vec{S}_1 \cdot \vec{S}_2 \vec{v}_1 \cdot \vec{v}_2 + 4 \vec{S}_1 \cdot \vec{S}_2 \vec{v}_2 \cdot \vec{v}_2 \right) + \frac{8 \vec{S}_1 \cdot \vec{S}_2 \hat{n} \cdot \vec{v}_1 - 8 \hat{n} \cdot \vec{S}_2 \hat{n} \cdot \vec{S}_1 \hat{n} \cdot \vec{v}_1}{r^4} \right) \Bigg\}$$

{DiagS1S2 [3, 7, 1],

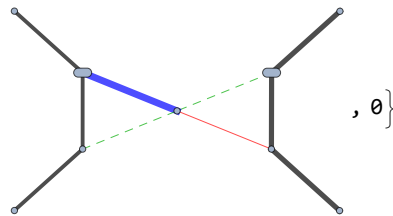



$\{\text{DiagS1S2}[3, 7, 2],$ 
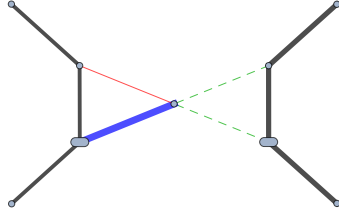
 $, 0\}$ 
 $\{\text{DiagS1S2}[3, 7, 3],$ 
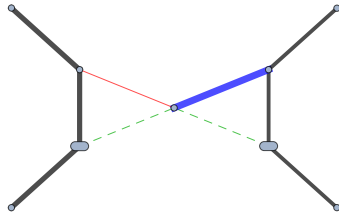
 $, \frac{1}{r^5}$ 

$$\pi^2 G^3 m_1 m_2 \left( -\frac{945}{16} \hat{n} \cdot \vec{S}_1 \hat{n} \cdot \vec{S}_2 (\hat{n} \cdot \vec{v}_2)^2 + \frac{135}{16} \vec{S}_1 \cdot \vec{S}_2 (\hat{n} \cdot \vec{v}_2)^2 + \frac{135}{8} \hat{n} \cdot \vec{S}_2 \hat{n} \cdot \vec{v}_2 \vec{S}_1 \cdot \vec{v}_2 + \right. \\ \left. \frac{135}{8} \hat{n} \cdot \vec{S}_1 \hat{n} \cdot \vec{v}_2 \vec{S}_2 \cdot \vec{v}_2 + \frac{135}{16} \vec{v}_2 \cdot \vec{v}_2 \hat{n} \cdot \vec{S}_1 \hat{n} \cdot \vec{S}_2 - \frac{27}{8} \vec{S}_1 \cdot \vec{v}_2 \vec{S}_2 \cdot \vec{v}_2 - \frac{27}{16} \vec{S}_1 \cdot \vec{S}_2 \vec{v}_2 \cdot \vec{v}_2 \right) \}$$

 $\{\text{DiagS1S2}[3, 7, 4],$ 
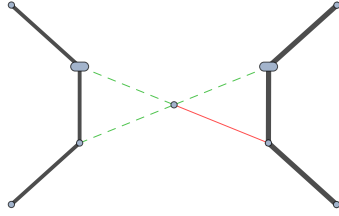
 $,$ 

$$\pi^2 G^3 m_1 m_2 \left( \frac{1}{r^5} \left( \frac{315}{8} \hat{n} \cdot \vec{S}_1 \hat{n} \cdot \vec{S}_2 (\hat{n} \cdot \vec{v}_2)^2 - \frac{45}{8} \vec{S}_1 \cdot \vec{S}_2 (\hat{n} \cdot \vec{v}_2)^2 + \frac{315}{4} \hat{n} \cdot \vec{S}_1 \hat{n} \cdot \vec{S}_2 \hat{n} \cdot \vec{v}_1 \hat{n} \cdot \vec{v}_2 - \frac{45}{4} \vec{S}_1 \cdot \vec{S}_2 \hat{n} \cdot \vec{v}_1 \hat{n} \cdot \vec{v}_2 - \right. \right. \\ \frac{45}{4} \hat{n} \cdot \vec{S}_2 \hat{n} \cdot \vec{v}_2 \vec{S}_1 \cdot \vec{v}_1 - \frac{45}{4} \hat{n} \cdot \vec{S}_2 \hat{n} \cdot \vec{v}_2 \vec{S}_1 \cdot \vec{v}_2 - \frac{45}{4} \hat{n} \cdot \vec{S}_1 \hat{n} \cdot \vec{v}_2 \vec{S}_2 \cdot \vec{v}_1 - \frac{45}{4} \hat{n} \cdot \vec{S}_1 \hat{n} \cdot \vec{v}_2 \vec{S}_2 \cdot \vec{v}_2 - \\ \frac{45}{4} \hat{n} \cdot \vec{S}_2 \hat{n} \cdot \vec{v}_1 \vec{S}_1 \cdot \vec{v}_2 - \frac{45}{4} \hat{n} \cdot \vec{S}_1 \hat{n} \cdot \vec{v}_1 \vec{S}_2 \cdot \vec{v}_2 - \frac{45}{4} \vec{v}_1 \cdot \vec{v}_2 \hat{n} \cdot \vec{S}_1 \hat{n} \cdot \vec{S}_2 - \frac{45}{8} \vec{v}_2 \cdot \vec{v}_2 \hat{n} \cdot \vec{S}_1 \hat{n} \cdot \vec{S}_2 + \\ \left. \frac{9}{4} \vec{S}_1 \cdot \vec{v}_2 \vec{S}_2 \cdot \vec{v}_1 + \frac{9}{4} \vec{S}_1 \cdot \vec{v}_1 \vec{S}_2 \cdot \vec{v}_2 + \frac{9}{4} \vec{S}_1 \cdot \vec{v}_2 \vec{S}_2 \cdot \vec{v}_2 + \frac{9}{4} \vec{S}_1 \cdot \vec{S}_2 \vec{v}_1 \cdot \vec{v}_2 + \frac{9}{8} \vec{S}_1 \cdot \vec{S}_2 \vec{v}_2 \cdot \vec{v}_2 \right) + \\ \frac{1}{r^4} \left( \frac{15}{2} \hat{n} \cdot \vec{S}_2 \hat{n} \cdot \vec{S}_1 \hat{n} \cdot \vec{v}_2 - 15 \hat{n} \cdot \vec{S}_1 \hat{n} \cdot \vec{S}_2 \hat{n} \cdot \vec{v}_2 + 3 \vec{S}_1 \cdot \vec{S}_2 \hat{n} \cdot \vec{v}_2 - \frac{3}{2} \vec{S}_1 \cdot \vec{S}_2 \hat{n} \cdot \vec{v}_2 + \right. \\ \left. 3 \hat{n} \cdot \vec{S}_2 \vec{S}_1 \cdot \vec{v}_2 - \frac{3}{2} \hat{n} \cdot \vec{S}_1 \vec{S}_2 \cdot \vec{v}_2 - \frac{3}{2} \hat{n} \cdot \vec{S}_2 \vec{S}_1 \cdot \vec{v}_2 + 3 \hat{n} \cdot \vec{S}_1 \vec{S}_2 \cdot \vec{v}_2 \right) \left. \right) \}$$

 $\{\text{DiagS1S2}[3, 7, 5],$ 
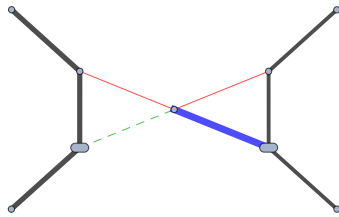
 $, \frac{1}{r^5}$ 

$$\pi^2 G^3 m_1 m_2 \left( -\frac{105}{64} \hat{n} \cdot \vec{S}_1 \hat{n} \cdot \vec{S}_2 (\hat{n} \cdot \vec{v}_2)^2 + \frac{15}{64} \vec{S}_1 \cdot \vec{S}_2 (\hat{n} \cdot \vec{v}_2)^2 - \frac{105}{64} \hat{n} \cdot \vec{S}_1 \hat{n} \cdot \vec{S}_2 \hat{n} \cdot \vec{v}_1 \hat{n} \cdot \vec{v}_2 + \frac{15}{64} \vec{S}_1 \cdot \vec{S}_2 \hat{n} \cdot \vec{v}_1 \hat{n} \cdot \vec{v}_2 + \right. \\ \frac{15}{64} \hat{n} \cdot \vec{S}_2 \hat{n} \cdot \vec{v}_2 \vec{S}_1 \cdot \vec{v}_1 + \frac{15}{32} \hat{n} \cdot \vec{S}_2 \hat{n} \cdot \vec{v}_2 \vec{S}_1 \cdot \vec{v}_2 + \frac{15}{64} \hat{n} \cdot \vec{S}_1 \hat{n} \cdot \vec{v}_2 \vec{S}_2 \cdot \vec{v}_1 + \frac{15}{32} \hat{n} \cdot \vec{S}_1 \hat{n} \cdot \vec{v}_2 \vec{S}_2 \cdot \vec{v}_2 + \\ \frac{15}{64} \hat{n} \cdot \vec{S}_2 \hat{n} \cdot \vec{v}_1 \vec{S}_1 \cdot \vec{v}_2 + \frac{15}{64} \hat{n} \cdot \vec{S}_1 \hat{n} \cdot \vec{v}_1 \vec{S}_2 \cdot \vec{v}_2 + \frac{15}{64} \vec{v}_1 \cdot \vec{v}_2 \hat{n} \cdot \vec{S}_1 \hat{n} \cdot \vec{S}_2 + \frac{15}{64} \vec{v}_2 \cdot \vec{v}_2 \hat{n} \cdot \vec{S}_1 \hat{n} \cdot \vec{S}_2 - \\ \left. \frac{3}{64} \vec{S}_1 \cdot \vec{v}_2 \vec{S}_2 \cdot \vec{v}_1 - \frac{3}{64} \vec{S}_1 \cdot \vec{v}_1 \vec{S}_2 \cdot \vec{v}_2 - \frac{3}{32} \vec{S}_1 \cdot \vec{v}_2 \vec{S}_2 \cdot \vec{v}_2 - \frac{3}{64} \vec{S}_1 \cdot \vec{S}_2 \vec{v}_1 \cdot \vec{v}_2 - \frac{3}{64} \vec{S}_1 \cdot \vec{S}_2 \vec{v}_2 \cdot \vec{v}_2 \right) \}$$

$$\left\{ \text{DiagS1S2}[3, 7, 6], \quad \theta \right\}$$
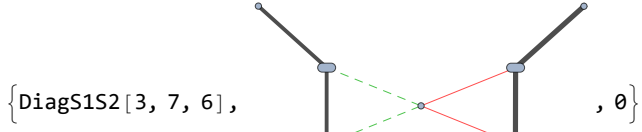

$$\left\{ \text{DiagS1S2}[3, 7, 7], \quad \theta \right\}$$
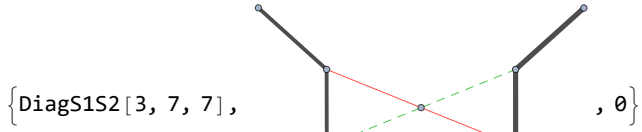

$$\left\{ \text{DiagS1S2}[3, 7, 8], \quad , \right\}$$
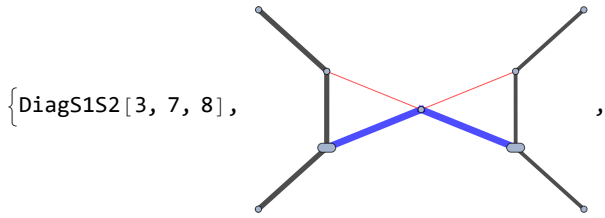

$$\frac{1}{r^5} \pi^2 G^3 m_1 m_2 \left( \frac{105}{32} \hat{n} \cdot \vec{S}_1 \hat{n} \cdot \vec{S}_2 \hat{n} \cdot \vec{v}_1 \hat{n} \cdot \vec{v}_2 - \frac{15}{32} \vec{S}_1 \cdot \vec{S}_2 \hat{n} \cdot \vec{v}_1 \hat{n} \cdot \vec{v}_2 - \frac{15}{32} \hat{n} \cdot \vec{S}_2 \hat{n} \cdot \vec{v}_2 \vec{S}_1 \cdot \vec{v}_1 - \frac{15}{32} \hat{n} \cdot \vec{S}_1 \hat{n} \cdot \vec{v}_2 \vec{S}_2 \cdot \vec{v}_1 - \frac{15}{32} \hat{n} \cdot \vec{S}_2 \hat{n} \cdot \vec{v}_1 \vec{S}_1 \cdot \vec{v}_2 - \frac{15}{32} \hat{n} \cdot \vec{S}_1 \hat{n} \cdot \vec{v}_1 \vec{S}_2 \cdot \vec{v}_2 - \frac{15}{32} \vec{v}_1 \cdot \vec{v}_2 \hat{n} \cdot \vec{S}_1 \hat{n} \cdot \vec{S}_2 + \frac{3}{32} \vec{S}_1 \cdot \vec{v}_2 \vec{S}_2 \cdot \vec{v}_1 + \frac{3}{32} \vec{S}_1 \cdot \vec{v}_1 \vec{S}_2 \cdot \vec{v}_2 + \frac{3}{32} \vec{S}_1 \cdot \vec{S}_2 \vec{v}_1 \cdot \vec{v}_2 \right) \Bigg\}$$

$$\left\{ \text{DiagS1S2}[3, 7, 9], \quad \pi^2 G^3 m_1 m_2 \right\}$$
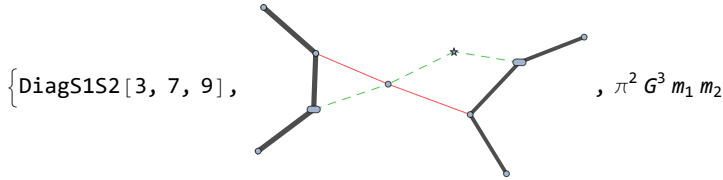

$$\left( \frac{1}{r^5} \left( \frac{735}{64} \hat{n} \cdot \vec{S}_1 \hat{n} \cdot \vec{S}_2 (\hat{n} \cdot \vec{v}_2)^2 - \frac{105}{64} \vec{S}_1 \cdot \vec{S}_2 (\hat{n} \cdot \vec{v}_2)^2 - \frac{315}{8} \hat{n} \cdot \vec{S}_1 \hat{n} \cdot \vec{S}_2 \hat{n} \cdot \vec{v}_1 \hat{n} \cdot \vec{v}_2 + \frac{45}{8} \vec{S}_1 \cdot \vec{S}_2 \hat{n} \cdot \vec{v}_1 \hat{n} \cdot \vec{v}_2 + \frac{45}{8} \hat{n} \cdot \vec{S}_2 \hat{n} \cdot \vec{v}_2 \vec{S}_1 \cdot \vec{v}_1 - \frac{105}{32} \hat{n} \cdot \vec{S}_2 \hat{n} \cdot \vec{v}_2 \vec{S}_1 \cdot \vec{v}_2 + \frac{45}{8} \hat{n} \cdot \vec{S}_1 \hat{n} \cdot \vec{v}_2 \vec{S}_2 \cdot \vec{v}_1 - \frac{105}{32} \hat{n} \cdot \vec{S}_1 \hat{n} \cdot \vec{v}_2 \vec{S}_2 \cdot \vec{v}_2 + \frac{45}{8} \hat{n} \cdot \vec{S}_2 \hat{n} \cdot \vec{v}_1 \vec{S}_1 \cdot \vec{v}_2 + \frac{45}{8} \hat{n} \cdot \vec{S}_1 \hat{n} \cdot \vec{v}_1 \vec{S}_2 \cdot \vec{v}_2 + \frac{45}{8} \vec{v}_1 \cdot \vec{v}_2 \hat{n} \cdot \vec{S}_1 \hat{n} \cdot \vec{S}_2 - \frac{105}{64} \vec{v}_2 \cdot \vec{v}_2 \hat{n} \cdot \vec{S}_1 \hat{n} \cdot \vec{S}_2 - \frac{9}{8} \vec{S}_1 \cdot \vec{v}_2 \vec{S}_2 \cdot \vec{v}_1 - \frac{9}{8} \vec{S}_1 \cdot \vec{v}_1 \vec{S}_2 \cdot \vec{v}_2 + \frac{21}{32} \vec{S}_1 \cdot \vec{v}_2 \vec{S}_2 \cdot \vec{v}_2 - \frac{9}{8} \vec{S}_1 \cdot \vec{S}_2 \vec{v}_1 \cdot \vec{v}_2 + \frac{21}{64} \vec{S}_1 \cdot \vec{S}_2 \vec{v}_2 \cdot \vec{v}_2 \right) + \frac{1}{r^4} \left( -\frac{105}{8} \hat{n} \cdot \vec{S}_2 \hat{n} \cdot \vec{S}_1 \hat{n} \cdot \vec{v}_1 + \frac{21}{8} \vec{S}_1 \cdot \vec{S}_2 \hat{n} \cdot \vec{v}_1 + \frac{15}{2} \hat{n} \cdot \vec{S}_2 \hat{n} \cdot \vec{S}_1 \hat{n} \cdot \vec{v}_2 + \frac{45}{8} \hat{n} \cdot \vec{S}_1 \hat{n} \cdot \vec{S}_2 \hat{n} \cdot \vec{v}_2 - \frac{9}{8} \vec{S}_1 \cdot \vec{S}_2 \hat{n} \cdot \vec{v}_2 - \frac{9}{8} \hat{n} \cdot \vec{S}_2 \vec{S}_1 \cdot \vec{v}_2 + \frac{21}{8} \hat{n} \cdot \vec{S}_1 \vec{S}_2 \cdot \vec{v}_1 - \frac{3}{2} \hat{n} \cdot \vec{S}_1 \vec{S}_2 \cdot \vec{v}_2 - \frac{3}{2} \vec{S}_1 \cdot \vec{S}_2 \hat{n} \cdot \vec{v}_2 + \frac{21}{8} \hat{n} \cdot \vec{S}_2 \vec{S}_1 \cdot \vec{v}_1 - \frac{3}{2} \hat{n} \cdot \vec{S}_2 \vec{S}_1 \cdot \vec{v}_2 - \frac{9}{8} \hat{n} \cdot \vec{S}_1 \vec{S}_2 \cdot \vec{v}_2 \right) + \frac{\frac{21}{8} \hat{n} \cdot \vec{S}_1 \hat{n} \cdot \vec{S}_2 - \frac{7}{8} \vec{S}_1 \cdot \vec{S}_2}{r^3} \right) \Bigg\}$$

$\{\text{DiagS1S2}[3, 7, 10],$ 
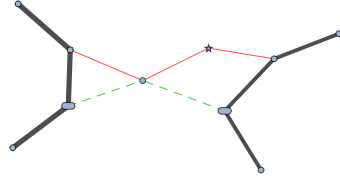
 $, \frac{1}{r^5}$ 

$$\pi^2 G^3 m_1 m_2 \left( -\frac{105}{64} \hat{n} \cdot \vec{S}_1 \hat{n} \cdot \vec{S}_2 (\hat{n} \cdot \vec{v}_2)^2 + \frac{15}{64} \vec{S}_1 \cdot \vec{S}_2 (\hat{n} \cdot \vec{v}_2)^2 + \frac{15}{32} \hat{n} \cdot \vec{S}_2 \hat{n} \cdot \vec{v}_2 \vec{S}_1 \cdot \vec{v}_2 + \right. \\ \left. \frac{15}{32} \hat{n} \cdot \vec{S}_1 \hat{n} \cdot \vec{v}_2 \vec{S}_2 \cdot \vec{v}_2 + \frac{15}{64} \vec{v}_2 \cdot \vec{v}_2 \hat{n} \cdot \vec{S}_1 \hat{n} \cdot \vec{S}_2 - \frac{3}{32} \vec{S}_1 \cdot \vec{v}_2 \vec{S}_2 \cdot \vec{v}_2 - \frac{3}{64} \vec{S}_1 \cdot \vec{S}_2 \vec{v}_2 \cdot \vec{v}_2 \right) \}$$

 $\{\text{DiagS1S2}[3, 7, 11],$ 
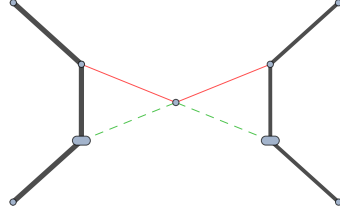
 $,$ 

$$\frac{1}{r^5} \pi^2 G^3 m_1 m_2 \left( \frac{105}{32} \hat{n} \cdot \vec{S}_1 \hat{n} \cdot \vec{S}_2 \hat{n} \cdot \vec{v}_1 \hat{n} \cdot \vec{v}_2 - \frac{15}{32} \vec{S}_1 \cdot \vec{S}_2 \hat{n} \cdot \vec{v}_1 \hat{n} \cdot \vec{v}_2 - \right. \\ \left. \frac{15}{32} \hat{n} \cdot \vec{S}_2 \hat{n} \cdot \vec{v}_2 \vec{S}_1 \cdot \vec{v}_1 - \frac{15}{32} \hat{n} \cdot \vec{S}_1 \hat{n} \cdot \vec{v}_2 \vec{S}_2 \cdot \vec{v}_1 - \frac{15}{32} \hat{n} \cdot \vec{S}_2 \hat{n} \cdot \vec{v}_1 \vec{S}_1 \cdot \vec{v}_2 - \frac{15}{32} \hat{n} \cdot \vec{S}_1 \hat{n} \cdot \vec{v}_1 \vec{S}_2 \cdot \vec{v}_2 - \right. \\ \left. \frac{15}{32} \vec{v}_1 \cdot \vec{v}_2 \hat{n} \cdot \vec{S}_1 \hat{n} \cdot \vec{S}_2 + \frac{3}{32} \vec{S}_1 \cdot \vec{v}_2 \vec{S}_2 \cdot \vec{v}_1 + \frac{3}{32} \vec{S}_1 \cdot \vec{v}_1 \vec{S}_2 \cdot \vec{v}_2 + \frac{3}{32} \vec{S}_1 \cdot \vec{S}_2 \vec{v}_1 \cdot \vec{v}_2 \right) \}$$

 $\{\text{DiagS1S2}[3, 8, 1],$ 
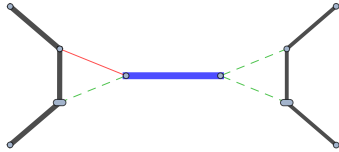
 $,$ 

$$\frac{\pi^2 G^3 m_1 m_2 \left( \frac{15}{16} \hat{n} \cdot \vec{S}_1 \hat{n} \cdot \vec{S}_2 \hat{n} \cdot \vec{v}_2 - \frac{3}{16} \vec{S}_1 \cdot \vec{S}_2 \hat{n} \cdot \vec{v}_2 - \frac{3}{16} \hat{n} \cdot \vec{S}_2 \vec{S}_1 \cdot \vec{v}_2 - \frac{3}{16} \hat{n} \cdot \vec{S}_1 \vec{S}_2 \cdot \vec{v}_2 \right)}{r^4} \}$$

 $\{\text{DiagS1S2}[3, 8, 2],$ 
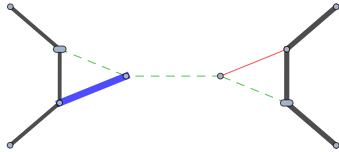
 $, \frac{1}{r^5}$ 

$$\pi^2 G^3 m_1 m_2 \left( \frac{315}{16} \hat{n} \cdot \vec{S}_1 \hat{n} \cdot \vec{S}_2 (\hat{n} \cdot \vec{v}_2)^2 - \frac{45}{16} \vec{S}_1 \cdot \vec{S}_2 (\hat{n} \cdot \vec{v}_2)^2 - \frac{45}{8} \hat{n} \cdot \vec{S}_2 \hat{n} \cdot \vec{v}_2 \vec{S}_1 \cdot \vec{v}_2 - \right. \\ \left. \frac{45}{8} \hat{n} \cdot \vec{S}_1 \hat{n} \cdot \vec{v}_2 \vec{S}_2 \cdot \vec{v}_2 - \frac{45}{16} \vec{v}_2 \cdot \vec{v}_2 \hat{n} \cdot \vec{S}_1 \hat{n} \cdot \vec{S}_2 + \frac{9}{8} \vec{S}_1 \cdot \vec{v}_2 \vec{S}_2 \cdot \vec{v}_2 + \frac{9}{16} \vec{S}_1 \cdot \vec{S}_2 \vec{v}_2 \cdot \vec{v}_2 \right) \}$$

 $\{\text{DiagS1S2}[3, 8, 3],$ 
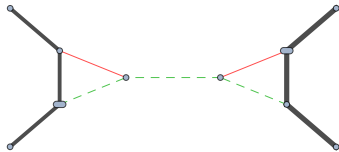
 $, \emptyset \}$ 
 $\{\text{DiagS1S2}[3, 8, 4],$ 
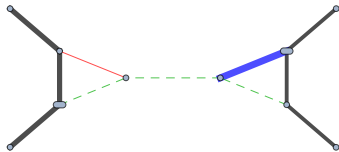
 $, \emptyset \}$

$\left\{ \text{DiagS1S2}[3, 8, 5], \right.$ 
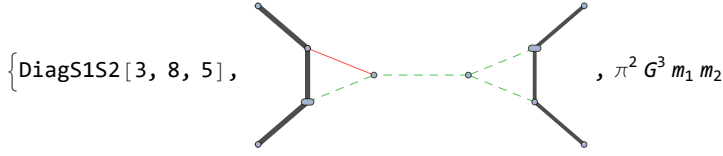
 $, \pi^2 G^3 m_1 m_2$

$$\begin{aligned}
 & \left( \frac{1}{r^5} \left( -\frac{315}{16} \hat{n} \cdot \vec{S}_1 \hat{n} \cdot \vec{S}_2 (\hat{n} \cdot \vec{v}_2)^2 + \frac{45}{16} \vec{S}_1 \cdot \vec{S}_2 (\hat{n} \cdot \vec{v}_2)^2 - \frac{315}{16} \hat{n} \cdot \vec{S}_1 \hat{n} \cdot \vec{S}_2 \hat{n} \cdot \vec{v}_1 \hat{n} \cdot \vec{v}_2 + \frac{45}{16} \vec{S}_1 \cdot \vec{S}_2 \hat{n} \cdot \vec{v}_1 \hat{n} \cdot \vec{v}_2 + \right. \right. \\
 & \quad \frac{45}{16} \hat{n} \cdot \vec{S}_2 \hat{n} \cdot \vec{v}_2 \vec{S}_1 \cdot \vec{v}_1 + \frac{45}{8} \hat{n} \cdot \vec{S}_2 \hat{n} \cdot \vec{v}_2 \vec{S}_1 \cdot \vec{v}_2 + \frac{45}{16} \hat{n} \cdot \vec{S}_1 \hat{n} \cdot \vec{v}_2 \vec{S}_2 \cdot \vec{v}_1 + \frac{45}{8} \hat{n} \cdot \vec{S}_1 \hat{n} \cdot \vec{v}_2 \vec{S}_2 \cdot \vec{v}_2 + \\
 & \quad \frac{45}{16} \hat{n} \cdot \vec{S}_2 \hat{n} \cdot \vec{v}_1 \vec{S}_1 \cdot \vec{v}_2 + \frac{45}{16} \hat{n} \cdot \vec{S}_1 \hat{n} \cdot \vec{v}_1 \vec{S}_2 \cdot \vec{v}_2 + \frac{45}{16} \vec{v}_1 \cdot \vec{v}_2 \hat{n} \cdot \vec{S}_1 \hat{n} \cdot \vec{S}_2 + \frac{45}{16} \vec{v}_2 \cdot \vec{v}_2 \hat{n} \cdot \vec{S}_1 \hat{n} \cdot \vec{S}_2 - \\
 & \quad \left. \frac{9}{16} \vec{S}_1 \cdot \vec{v}_2 \vec{S}_2 \cdot \vec{v}_1 - \frac{9}{16} \vec{S}_1 \cdot \vec{v}_1 \vec{S}_2 \cdot \vec{v}_2 - \frac{9}{8} \vec{S}_1 \cdot \vec{v}_2 \vec{S}_2 \cdot \vec{v}_2 - \frac{9}{16} \vec{S}_1 \cdot \vec{S}_2 \vec{v}_1 \cdot \vec{v}_2 - \frac{9}{16} \vec{S}_1 \cdot \vec{S}_2 \vec{v}_2 \cdot \vec{v}_2 \right) + \\
 & \quad \frac{1}{r^4} \left( -\frac{15}{4} \hat{n} \cdot \vec{S}_2 \hat{n} \cdot \vec{S}_1 \hat{n} \cdot \vec{v}_2 + \frac{45}{16} \hat{n} \cdot \vec{S}_1 \hat{n} \cdot \vec{S}_2 \hat{n} \cdot \vec{v}_2 - \frac{9}{16} \vec{S}_1 \cdot \vec{S}_2 \hat{n} \cdot \vec{v}_2 + \frac{3}{4} \vec{S}_1 \cdot \vec{S}_2 \hat{n} \cdot \vec{v}_2 - \right. \\
 & \quad \left. \frac{9}{16} \hat{n} \cdot \vec{S}_2 \vec{S}_1 \cdot \vec{v}_2 + \frac{3}{4} \hat{n} \cdot \vec{S}_1 \vec{S}_2 \cdot \vec{v}_2 + \frac{3}{4} \hat{n} \cdot \vec{S}_2 \vec{S}_1 \cdot \vec{v}_2 - \frac{9}{16} \hat{n} \cdot \vec{S}_1 \vec{S}_2 \cdot \vec{v}_2 \right) \Bigg\}
 \end{aligned}$$

$\left\{ \text{DiagS1S2}[3, 8, 6], \right.$ 
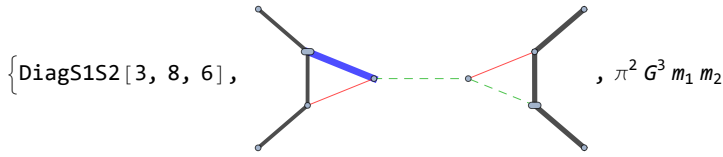
 $, \pi^2 G^3 m_1 m_2$

$$\begin{aligned}
 & \left( \frac{1}{r^5} \left( -\frac{105}{16} \hat{n} \cdot \vec{S}_1 \hat{n} \cdot \vec{S}_2 (\hat{n} \cdot \vec{v}_2)^2 + \frac{15}{16} \vec{S}_1 \cdot \vec{S}_2 (\hat{n} \cdot \vec{v}_2)^2 + \frac{105}{16} \hat{n} \cdot \vec{S}_1 \hat{n} \cdot \vec{S}_2 \hat{n} \cdot \vec{v}_1 \hat{n} \cdot \vec{v}_2 - \frac{15}{16} \vec{S}_1 \cdot \vec{S}_2 \hat{n} \cdot \vec{v}_1 \hat{n} \cdot \vec{v}_2 - \right. \right. \\
 & \quad \frac{15}{16} \hat{n} \cdot \vec{S}_2 \hat{n} \cdot \vec{v}_2 \vec{S}_1 \cdot \vec{v}_1 + \frac{15}{8} \hat{n} \cdot \vec{S}_2 \hat{n} \cdot \vec{v}_2 \vec{S}_1 \cdot \vec{v}_2 - \frac{15}{16} \hat{n} \cdot \vec{S}_1 \hat{n} \cdot \vec{v}_2 \vec{S}_2 \cdot \vec{v}_1 + \frac{15}{8} \hat{n} \cdot \vec{S}_1 \hat{n} \cdot \vec{v}_2 \vec{S}_2 \cdot \vec{v}_2 - \\
 & \quad \frac{15}{16} \hat{n} \cdot \vec{S}_2 \hat{n} \cdot \vec{v}_1 \vec{S}_1 \cdot \vec{v}_2 - \frac{15}{16} \hat{n} \cdot \vec{S}_1 \hat{n} \cdot \vec{v}_1 \vec{S}_2 \cdot \vec{v}_2 - \frac{15}{16} \vec{v}_1 \cdot \vec{v}_2 \hat{n} \cdot \vec{S}_1 \hat{n} \cdot \vec{S}_2 + \frac{15}{16} \vec{v}_2 \cdot \vec{v}_2 \hat{n} \cdot \vec{S}_1 \hat{n} \cdot \vec{S}_2 + \\
 & \quad \frac{3}{16} \vec{S}_1 \cdot \vec{v}_2 \vec{S}_2 \cdot \vec{v}_1 + \frac{3}{16} \vec{S}_1 \cdot \vec{v}_1 \vec{S}_2 \cdot \vec{v}_2 - \frac{3}{8} \vec{S}_1 \cdot \vec{v}_2 \vec{S}_2 \cdot \vec{v}_2 + \frac{3}{16} \vec{S}_1 \cdot \vec{S}_2 \vec{v}_1 \cdot \vec{v}_2 - \frac{3}{16} \vec{S}_1 \cdot \vec{S}_2 \vec{v}_2 \cdot \vec{v}_2 \Bigg) + \\
 & \quad \left. \frac{-\frac{15}{16} \hat{n} \cdot \vec{S}_1 \hat{n} \cdot \vec{S}_2 \hat{n} \cdot \vec{v}_2 + \frac{3}{16} \vec{S}_1 \cdot \vec{S}_2 \hat{n} \cdot \vec{v}_2 + \frac{3}{16} \hat{n} \cdot \vec{S}_2 \vec{S}_1 \cdot \vec{v}_2 + \frac{3}{16} \hat{n} \cdot \vec{S}_1 \vec{S}_2 \cdot \vec{v}_2}{r^4} \right\}
 \end{aligned}$$

$\left\{ \text{DiagS1S2}[3, 8, 7], \right.$ 
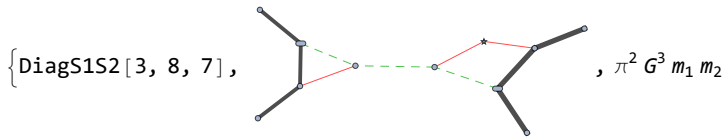
 $, \pi^2 G^3 m_1 m_2$

$$\begin{aligned}
 & \left( \frac{1}{r^5} \left( -\frac{315}{64} \hat{n} \cdot \vec{S}_1 \hat{n} \cdot \vec{S}_2 (\hat{n} \cdot \vec{v}_1)^2 + \frac{45}{64} \vec{S}_1 \cdot \vec{S}_2 (\hat{n} \cdot \vec{v}_1)^2 + \frac{105}{16} \hat{n} \cdot \vec{S}_1 \hat{n} \cdot \vec{S}_2 \hat{n} \cdot \vec{v}_2 \hat{n} \cdot \vec{v}_1 - \frac{15}{16} \vec{S}_1 \cdot \vec{S}_2 \hat{n} \cdot \vec{v}_2 \hat{n} \cdot \vec{v}_1 + \right. \right. \\
 & \quad \frac{45}{32} \hat{n} \cdot \vec{S}_2 \hat{n} \cdot \vec{v}_1 \vec{S}_1 \cdot \vec{v}_1 - \frac{15}{16} \hat{n} \cdot \vec{S}_2 \hat{n} \cdot \vec{v}_1 \vec{S}_1 \cdot \vec{v}_2 + \frac{45}{32} \hat{n} \cdot \vec{S}_1 \hat{n} \cdot \vec{v}_1 \vec{S}_2 \cdot \vec{v}_1 - \frac{15}{16} \hat{n} \cdot \vec{S}_1 \hat{n} \cdot \vec{v}_1 \vec{S}_2 \cdot \vec{v}_2 - \\
 & \quad \frac{15}{16} \hat{n} \cdot \vec{S}_2 \hat{n} \cdot \vec{v}_2 \vec{S}_1 \cdot \vec{v}_1 - \frac{15}{16} \hat{n} \cdot \vec{S}_1 \hat{n} \cdot \vec{v}_2 \vec{S}_2 \cdot \vec{v}_1 + \frac{45}{64} \vec{v}_1 \cdot \vec{v}_1 \hat{n} \cdot \vec{S}_1 \hat{n} \cdot \vec{S}_2 - \frac{15}{16} \vec{v}_1 \cdot \vec{v}_2 \hat{n} \cdot \vec{S}_1 \hat{n} \cdot \vec{S}_2 - \\
 & \quad \frac{9}{32} \vec{S}_1 \cdot \vec{v}_1 \vec{S}_2 \cdot \vec{v}_1 + \frac{3}{16} \vec{S}_1 \cdot \vec{v}_2 \vec{S}_2 \cdot \vec{v}_1 + \frac{3}{16} \vec{S}_1 \cdot \vec{v}_1 \vec{S}_2 \cdot \vec{v}_2 - \frac{9}{64} \vec{S}_1 \cdot \vec{S}_2 \vec{v}_1 \cdot \vec{v}_1 + \frac{3}{16} \vec{S}_1 \cdot \vec{S}_2 \vec{v}_1 \cdot \vec{v}_2 \Bigg) + \\
 & \quad \frac{1}{r^4} \left( \frac{15}{16} \hat{n} \cdot \vec{S}_2 \hat{n} \cdot \vec{S}_1 \hat{n} \cdot \vec{v}_1 + \frac{15}{16} \hat{n} \cdot \vec{S}_1 \hat{n} \cdot \vec{S}_2 \hat{n} \cdot \vec{v}_1 - \frac{3}{16} \vec{S}_1 \cdot \vec{S}_2 \hat{n} \cdot \vec{v}_1 - \frac{3}{16} \vec{S}_1 \cdot \vec{S}_2 \hat{n} \cdot \vec{v}_1 - \right.
 \end{aligned}$$

$$\left. \left. \left. \frac{3}{16} \hat{n} \cdot \vec{S}_2 \vec{S}_1 \cdot \vec{v}_1 - \frac{3}{16} \hat{n} \cdot \vec{S}_1 \vec{S}_2 \cdot \vec{v}_1 - \frac{3}{16} \hat{n} \cdot \vec{S}_2 \vec{S}_1 \cdot \vec{v}_1 - \frac{3}{16} \hat{n} \cdot \vec{S}_1 \vec{S}_2 \cdot \vec{v}_1 \right) \right) \right\}$$

$$\left\{ \text{DiagS1S2}[3, 8, 8], \pi^2 G^3 m_1 m_2 \right.$$
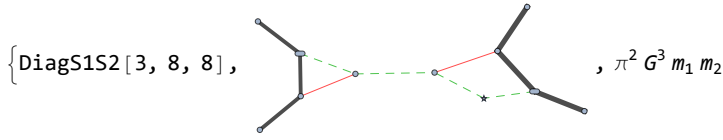

$$\left( \frac{1}{r^5} \left( -\frac{315}{64} \hat{n} \cdot \vec{S}_1 \hat{n} \cdot \vec{S}_2 (\hat{n} \cdot \vec{v}_1)^2 + \frac{45}{64} \vec{S}_1 \cdot \vec{S}_2 (\hat{n} \cdot \vec{v}_1)^2 + \frac{315}{16} \hat{n} \cdot \vec{S}_1 \hat{n} \cdot \vec{S}_2 \hat{n} \cdot \vec{v}_2 \hat{n} \cdot \vec{v}_1 - \frac{45}{16} \vec{S}_1 \cdot \vec{S}_2 \hat{n} \cdot \vec{v}_2 \hat{n} \cdot \vec{v}_1 + \right. \right.$$

$$\frac{45}{32} \hat{n} \cdot \vec{S}_2 \hat{n} \cdot \vec{v}_1 \vec{S}_1 \cdot \vec{v}_1 - \frac{45}{16} \hat{n} \cdot \vec{S}_2 \hat{n} \cdot \vec{v}_1 \vec{S}_1 \cdot \vec{v}_2 + \frac{45}{32} \hat{n} \cdot \vec{S}_1 \hat{n} \cdot \vec{v}_1 \vec{S}_2 \cdot \vec{v}_1 - \frac{45}{16} \hat{n} \cdot \vec{S}_1 \hat{n} \cdot \vec{v}_1 \vec{S}_2 \cdot \vec{v}_2 -$$

$$\frac{45}{16} \hat{n} \cdot \vec{S}_2 \hat{n} \cdot \vec{v}_2 \vec{S}_1 \cdot \vec{v}_1 - \frac{45}{16} \hat{n} \cdot \vec{S}_1 \hat{n} \cdot \vec{v}_2 \vec{S}_2 \cdot \vec{v}_1 + \frac{45}{64} \vec{v}_1 \cdot \vec{v}_1 \hat{n} \cdot \vec{S}_1 \hat{n} \cdot \vec{S}_2 - \frac{45}{16} \vec{v}_1 \cdot \vec{v}_2 \hat{n} \cdot \vec{S}_1 \hat{n} \cdot \vec{S}_2 -$$

$$\frac{9}{32} \vec{S}_1 \cdot \vec{v}_1 \vec{S}_2 \cdot \vec{v}_1 + \frac{9}{16} \vec{S}_1 \cdot \vec{v}_2 \vec{S}_2 \cdot \vec{v}_1 + \frac{9}{16} \vec{S}_1 \cdot \vec{v}_1 \vec{S}_2 \cdot \vec{v}_2 - \frac{9}{64} \vec{S}_1 \cdot \vec{S}_2 \vec{v}_1 \cdot \vec{v}_1 + \frac{9}{16} \vec{S}_1 \cdot \vec{S}_2 \vec{v}_1 \cdot \vec{v}_2 \Big) +$$

$$\frac{1}{r^4} \left( \frac{45}{16} \hat{n} \cdot \vec{S}_2 \hat{n} \cdot \vec{S}_1 \hat{n} \cdot \vec{v}_1 + \frac{45}{16} \hat{n} \cdot \vec{S}_1 \hat{n} \cdot \vec{S}_2 \hat{n} \cdot \vec{v}_1 - \frac{9}{16} \vec{S}_1 \cdot \vec{S}_2 \hat{n} \cdot \vec{v}_1 - \frac{9}{16} \vec{S}_1 \cdot \vec{S}_2 \hat{n} \cdot \vec{v}_1 - \right.$$

$$\frac{45}{8} \hat{n} \cdot \vec{S}_1 \hat{n} \cdot \vec{S}_2 \hat{n} \cdot \vec{v}_2 + \frac{9}{8} \vec{S}_1 \cdot \vec{S}_2 \hat{n} \cdot \vec{v}_2 - \frac{9}{16} \hat{n} \cdot \vec{S}_2 \vec{S}_1 \cdot \vec{v}_1 + \frac{9}{8} \hat{n} \cdot \vec{S}_2 \vec{S}_1 \cdot \vec{v}_2 - \frac{9}{16} \hat{n} \cdot \vec{S}_1 \vec{S}_2 \cdot \vec{v}_1 -$$

$$\left. \left. \frac{9}{16} \hat{n} \cdot \vec{S}_2 \vec{S}_1 \cdot \vec{v}_1 - \frac{9}{16} \hat{n} \cdot \vec{S}_1 \vec{S}_2 \cdot \vec{v}_1 + \frac{9}{8} \hat{n} \cdot \vec{S}_1 \vec{S}_2 \cdot \vec{v}_2 \right) + \frac{\frac{3}{8} \vec{S}_1 \cdot \vec{S}_2 - \frac{9}{8} \hat{n} \cdot \vec{S}_1 \hat{n} \cdot \vec{S}_2}{r^3} \right\}$$

$$\left\{ \text{DiagS1S2}[3, 8, 9], \right.$$
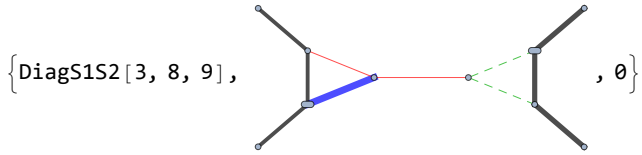

$$, \emptyset \}$$

$$\left\{ \text{DiagS1S2}[3, 8, 10], \right.$$
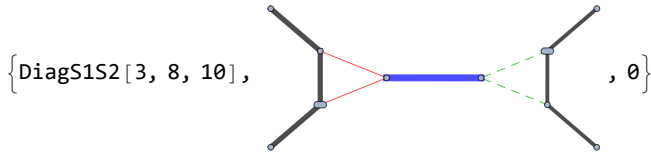

$$, \emptyset \}$$

$$\left\{ \text{DiagS1S2}[3, 8, 11], \right.$$
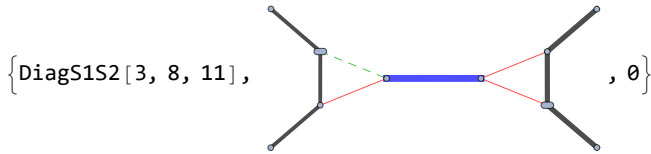

$$, \emptyset \}$$

$$\left\{ \text{DiagS1S2}[3, 8, 12], \right.$$
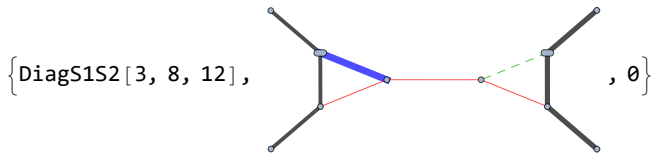

$$, \emptyset \}$$

$$\left\{ \text{DiagS1S2}[3, 8, 13], \right.$$
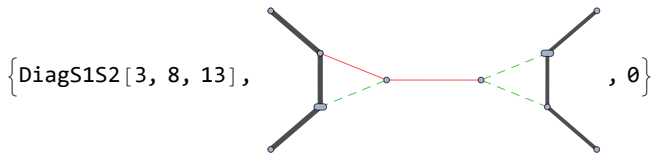

$$, \emptyset \}$$

$$\left\{ \text{DiagS1S2}[3, 8, 14], \right. , \left. \theta \right\}$$
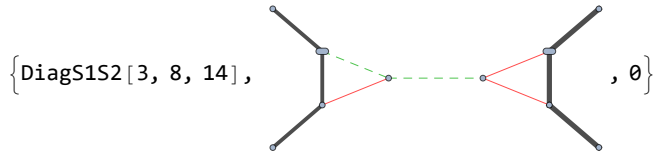

$$\left\{ \text{DiagS1S2}[3, 8, 15], \right. , \left. \theta \right\}$$
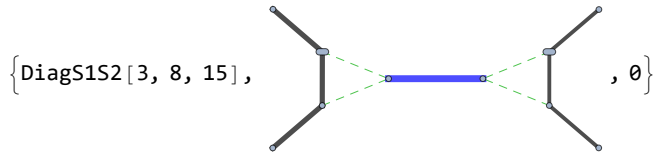

$$\left\{ \text{DiagS1S2}[3, 8, 16], \right. , \left. \frac{\pi^2 G^3 m_1 m_2 \left( \frac{3}{16} \hat{n} \cdot \vec{S}_1 \hat{n} \cdot \vec{S}_2 - \frac{1}{16} \vec{S}_1 \cdot \vec{S}_2 \right)}{r^3} \right\}$$
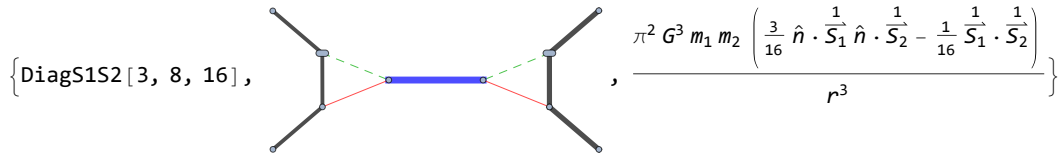

$$\left\{ \text{DiagS1S2}[3, 8, 17], \right. , \left. \theta \right\}$$
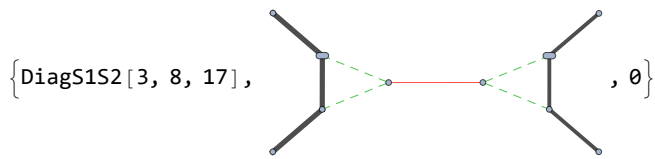

$$\left\{ \text{DiagS1S2}[3, 8, 18], \right. , \left. \theta \right\}$$
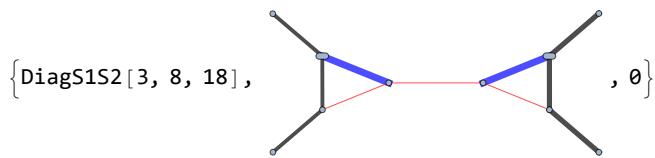

$$\left\{ \text{DiagS1S2}[3, 8, 19], \right. , \left. \theta \right\}$$
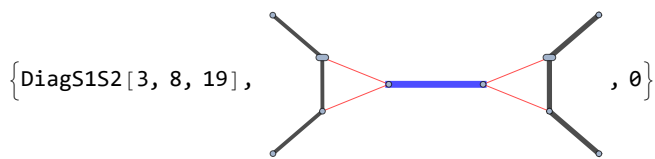

$$\left\{ \text{DiagS1S2}[3, 8, 20], \right. , \left. \theta \right\}$$
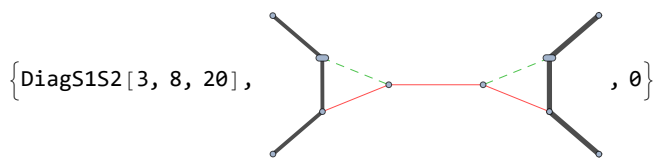

$$\left\{ \text{DiagS1S2}[3, 8, 21], \right. ,$$
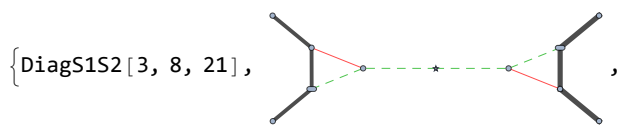

$$\pi^2 G^3 m_1 m_2 \left( \frac{1}{r^5} \left( \frac{105}{16} \hat{n} \cdot \vec{S}_1 \hat{n} \cdot \vec{S}_2 \hat{n} \cdot \vec{v}_1 \hat{n} \cdot \vec{v}_2 - \frac{15}{16} \vec{S}_1 \cdot \vec{S}_2 \hat{n} \cdot \vec{v}_1 \hat{n} \cdot \vec{v}_2 - \right. \right.$$

$$\frac{15}{16} \hat{n} \cdot \vec{S}_2 \hat{n} \cdot \vec{v}_2 \vec{S}_1 \cdot \vec{v}_1 - \frac{15}{16} \hat{n} \cdot \vec{S}_1 \hat{n} \cdot \vec{v}_2 \vec{S}_2 \cdot \vec{v}_1 - \frac{15}{16} \hat{n} \cdot \vec{S}_2 \hat{n} \cdot \vec{v}_1 \vec{S}_1 \cdot \vec{v}_2 - \frac{15}{16} \hat{n} \cdot \vec{S}_1 \hat{n} \cdot \vec{v}_1 \vec{S}_2 \cdot \vec{v}_2 -$$

$$\left. \frac{15}{16} \vec{v}_1 \cdot \vec{v}_2 \hat{n} \cdot \vec{S}_1 \hat{n} \cdot \vec{S}_2 + \frac{3}{16} \vec{S}_1 \cdot \vec{v}_2 \vec{S}_2 \cdot \vec{v}_1 + \frac{3}{16} \vec{S}_1 \cdot \vec{v}_1 \vec{S}_2 \cdot \vec{v}_2 + \frac{3}{16} \vec{S}_1 \cdot \vec{S}_2 \vec{v}_1 \cdot \vec{v}_2 \right) + \frac{1}{r^4}$$

$$\left( \frac{15}{16} \hat{n} \cdot \vec{S}_2 \hat{n} \cdot \vec{S}_1 \hat{n} \cdot \vec{v}_1 - \frac{3}{16} \vec{S}_1 \cdot \vec{S}_2 \hat{n} \cdot \vec{v}_1 - \frac{15}{16} \hat{n} \cdot \vec{S}_1 \hat{n} \cdot \vec{S}_2 \hat{n} \cdot \vec{v}_2 + \frac{3}{16} \vec{S}_1 \cdot \vec{S}_2 \hat{n} \cdot \vec{v}_2 + \frac{3}{16} \hat{n} \cdot \vec{S}_2 \vec{S}_1 \cdot \vec{v}_2 - \right.$$

$$\left. \left. \frac{3}{16} \hat{n} \cdot \vec{S}_1 \vec{S}_2 \cdot \vec{v}_1 - \frac{3}{16} \hat{n} \cdot \vec{S}_2 \vec{S}_1 \cdot \vec{v}_1 + \frac{3}{16} \hat{n} \cdot \vec{S}_1 \vec{S}_2 \cdot \vec{v}_2 \right) + \frac{\frac{1}{16} \vec{S}_1 \cdot \vec{S}_2 - \frac{3}{16} \hat{n} \cdot \vec{S}_1 \hat{n} \cdot \vec{S}_2}{r^3} \right\}$$

$$\left\{ \text{DiagS1S2}[3, 8, 22], \quad \emptyset \right\}$$
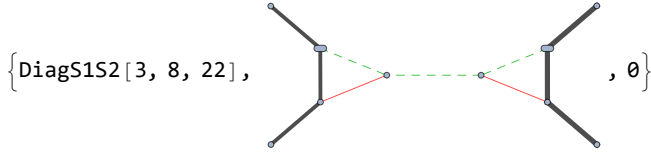

$$\left\{ \text{DiagS1S2}[3, 9, 1], \quad \frac{1}{r^5} \right\}$$
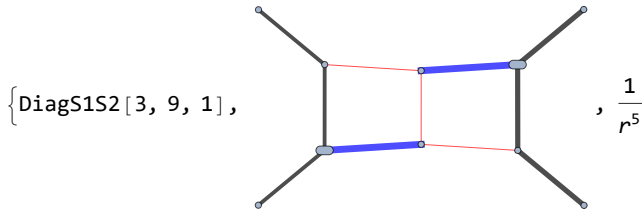

$$G^3 m_1 m_2 \left( -\frac{7}{4} \hat{n} \times \vec{S}_1 \cdot \vec{v}_2 \hat{n} \times \vec{S}_2 \cdot \vec{v}_1 - \frac{7}{4} \hat{n} \times \vec{S}_1 \cdot \vec{v}_1 \hat{n} \times \vec{S}_2 \cdot \vec{v}_2 - \frac{51}{4} \hat{n} \cdot \vec{S}_1 \hat{n} \cdot \vec{S}_2 \hat{n} \cdot \vec{v}_1 \hat{n} \cdot \vec{v}_2 + \frac{31}{4} \vec{S}_1 \cdot \vec{S}_2 \hat{n} \cdot \vec{v}_1 \hat{n} \cdot \vec{v}_2 + \right. \\ \left. \frac{5}{2} \hat{n} \cdot \vec{S}_2 \hat{n} \cdot \vec{v}_1 \vec{S}_1 \cdot \vec{v}_2 + \frac{5}{2} \hat{n} \cdot \vec{S}_1 \hat{n} \cdot \vec{v}_2 \vec{S}_2 \cdot \vec{v}_1 + \frac{7}{4} \vec{v}_1 \cdot \vec{v}_2 \hat{n} \cdot \vec{S}_1 \hat{n} \cdot \vec{S}_2 - \vec{S}_1 \cdot \vec{v}_2 \vec{S}_2 \cdot \vec{v}_1 - \frac{3}{4} \vec{S}_1 \cdot \vec{S}_2 \vec{v}_1 \cdot \vec{v}_2 \right) \Bigg\}$$

$$\left\{ \text{DiagS1S2}[3, 9, 2], \quad \right\}$$
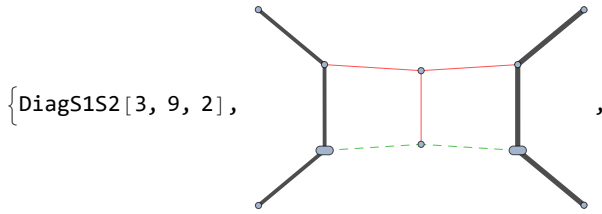

$$G^3 \left( \frac{1}{r^4} \left( 26 \hat{n} \cdot \vec{S}_2 \hat{n} \cdot \vec{S}_1 \hat{n} \cdot \vec{v}_1 + 26 \hat{n} \cdot \vec{S}_1 \hat{n} \cdot \vec{S}_2 \hat{n} \cdot \vec{v}_1 - 12 \vec{S}_1 \cdot \vec{S}_2 \hat{n} \cdot \vec{v}_1 - 12 \vec{S}_1 \cdot \vec{S}_2 \hat{n} \cdot \vec{v}_1 - 26 \hat{n} \cdot \vec{S}_2 \hat{n} \cdot \vec{S}_1 \hat{n} \cdot \vec{v}_2 - \right. \right. \\ \left. 26 \hat{n} \cdot \vec{S}_1 \hat{n} \cdot \vec{S}_2 \hat{n} \cdot \vec{v}_2 + 12 \hat{n} \cdot \vec{v}_2 \vec{S}_1 \cdot \vec{S}_2 + 2 \hat{n} \cdot \vec{S}_2 \vec{S}_1 \cdot \vec{v}_1 - 4 \hat{n} \cdot \vec{S}_2 \vec{S}_1 \cdot \vec{v}_2 + 4 \hat{n} \cdot \vec{S}_1 \vec{S}_2 \cdot \vec{v}_1 - \right. \\ \left. 2 \hat{n} \cdot \vec{S}_1 \vec{S}_2 \cdot \vec{v}_2 + 12 \hat{n} \cdot \vec{v}_2 \vec{S}_1 \cdot \vec{S}_2 + 2 \hat{n} \cdot \vec{S}_2 \vec{S}_1 \cdot \vec{v}_1 - 4 \hat{n} \cdot \vec{S}_2 \vec{S}_1 \cdot \vec{v}_2 + 4 \hat{n} \cdot \vec{S}_1 \vec{S}_2 \cdot \vec{v}_1 - 2 \hat{n} \cdot \vec{S}_1 \vec{S}_2 \cdot \vec{v}_2 \right) + \frac{1}{r^5} \\ \left( -152 \hat{n} \cdot \vec{S}_1 \hat{n} \cdot \vec{S}_2 (\hat{n} \cdot \vec{v}_1)^2 + 30 \vec{S}_1 \cdot \vec{S}_2 (\hat{n} \cdot \vec{v}_1)^2 + 332 \hat{n} \cdot \vec{S}_1 \hat{n} \cdot \vec{S}_2 \hat{n} \cdot \vec{v}_2 \hat{n} \cdot \vec{v}_1 - 98 \hat{n} \cdot \vec{v}_2 \vec{S}_1 \cdot \vec{S}_2 \hat{n} \cdot \vec{v}_1 + \right. \\ \left. 28 \hat{n} \cdot \vec{S}_2 \vec{S}_1 \cdot \vec{v}_1 \hat{n} \cdot \vec{v}_1 - 11 \hat{n} \cdot \vec{S}_2 \vec{S}_1 \cdot \vec{v}_2 \hat{n} \cdot \vec{v}_1 + 30 \hat{n} \cdot \vec{S}_1 \vec{S}_2 \cdot \vec{v}_1 \hat{n} \cdot \vec{v}_1 - 23 \hat{n} \cdot \vec{S}_1 \vec{S}_2 \cdot \vec{v}_2 \hat{n} \cdot \vec{v}_1 - \right. \\ \left. 152 \hat{n} \cdot \vec{S}_1 \hat{n} \cdot \vec{S}_2 (\hat{n} \cdot \vec{v}_2)^2 - 8 \hat{n} \times \vec{S}_1 \cdot \vec{v}_1 \hat{n} \times \vec{S}_2 \cdot \vec{v}_1 + 3 \hat{n} \times \vec{S}_1 \cdot \vec{v}_2 \hat{n} \times \vec{S}_2 \cdot \vec{v}_1 + 3 \hat{n} \times \vec{S}_1 \cdot \vec{v}_1 \hat{n} \times \vec{S}_2 \cdot \vec{v}_2 - \right. \\ \left. 8 \hat{n} \times \vec{S}_1 \cdot \vec{v}_2 \hat{n} \times \vec{S}_2 \cdot \vec{v}_2 + 30 (\hat{n} \cdot \vec{v}_2)^2 \vec{S}_1 \cdot \vec{S}_2 - 23 \hat{n} \cdot \vec{S}_2 \hat{n} \cdot \vec{v}_2 \vec{S}_1 \cdot \vec{v}_1 + 30 \hat{n} \cdot \vec{S}_2 \hat{n} \cdot \vec{v}_2 \vec{S}_1 \cdot \vec{v}_2 - 11 \hat{n} \cdot \vec{S}_1 \hat{n} \cdot \vec{v}_2 \vec{S}_2 \cdot \vec{v}_1 - \right. \\ \left. 2 \vec{S}_1 \cdot \vec{v}_1 \vec{S}_2 \cdot \vec{v}_1 - 5 \vec{S}_1 \cdot \vec{v}_2 \vec{S}_2 \cdot \vec{v}_1 + 28 \hat{n} \cdot \vec{S}_1 \hat{n} \cdot \vec{v}_2 \vec{S}_2 \cdot \vec{v}_2 - \vec{S}_1 \cdot \vec{v}_1 \vec{S}_2 \cdot \vec{v}_2 - 2 \vec{S}_1 \cdot \vec{v}_2 \vec{S}_2 \cdot \vec{v}_2 - 4 \hat{n} \cdot \vec{S}_1 \hat{n} \cdot \vec{S}_2 \vec{v}_1 \cdot \vec{v}_1 + \right. \\ \left. 6 \vec{S}_1 \cdot \vec{S}_2 \vec{v}_1 \cdot \vec{v}_1 - 26 \hat{n} \cdot \vec{S}_1 \hat{n} \cdot \vec{S}_2 \vec{v}_1 \cdot \vec{v}_2 + 10 \vec{S}_1 \cdot \vec{S}_2 \vec{v}_1 \cdot \vec{v}_2 - 4 \hat{n} \cdot \vec{S}_1 \hat{n} \cdot \vec{S}_2 \vec{v}_2 \cdot \vec{v}_2 + 6 \vec{S}_1 \cdot \vec{S}_2 \vec{v}_2 \cdot \vec{v}_2 \right) + \\ \pi^2 \left( \frac{1}{r^4} \left( \frac{15}{8} \hat{n} \cdot \vec{S}_2 \hat{n} \cdot \vec{S}_1 \hat{n} \cdot \vec{v}_1 + \frac{15}{8} \hat{n} \cdot \vec{S}_1 \hat{n} \cdot \vec{S}_2 \hat{n} \cdot \vec{v}_1 - \frac{3}{8} \vec{S}_1 \cdot \vec{S}_2 \hat{n} \cdot \vec{v}_1 - \frac{3}{8} \vec{S}_1 \cdot \vec{S}_2 \hat{n} \cdot \vec{v}_1 - \frac{15}{8} \hat{n} \cdot \vec{S}_2 \hat{n} \cdot \vec{S}_1 \hat{n} \cdot \vec{v}_2 - \right. \right. \\ \left. \frac{15}{8} \hat{n} \cdot \vec{S}_1 \hat{n} \cdot \vec{S}_2 \hat{n} \cdot \vec{v}_2 + \frac{3}{8} \hat{n} \cdot \vec{v}_2 \vec{S}_1 \cdot \vec{S}_2 - \frac{3}{8} \hat{n} \cdot \vec{S}_2 \vec{S}_1 \cdot \vec{v}_1 + \frac{3}{8} \hat{n} \cdot \vec{S}_2 \vec{S}_1 \cdot \vec{v}_2 - \frac{3}{8} \hat{n} \cdot \vec{S}_1 \vec{S}_2 \cdot \vec{v}_1 + \right. \\ \left. \frac{3}{8} \hat{n} \cdot \vec{S}_1 \vec{S}_2 \cdot \vec{v}_2 + \frac{3}{8} \hat{n} \cdot \vec{v}_2 \vec{S}_1 \cdot \vec{S}_2 - \frac{3}{8} \hat{n} \cdot \vec{S}_2 \vec{S}_1 \cdot \vec{v}_1 + \frac{3}{8} \hat{n} \cdot \vec{S}_2 \vec{S}_1 \cdot \vec{v}_2 - \frac{3}{8} \hat{n} \cdot \vec{S}_1 \vec{S}_2 \cdot \vec{v}_1 + \frac{3}{8} \hat{n} \cdot \vec{S}_1 \vec{S}_2 \cdot \vec{v}_2 \right) + \\ \left. \frac{1}{r^5} \left( -\frac{105}{16} \hat{n} \cdot \vec{S}_1 \hat{n} \cdot \vec{S}_2 (\hat{n} \cdot \vec{v}_1)^2 + \frac{15}{16} \vec{S}_1 \cdot \vec{S}_2 (\hat{n} \cdot \vec{v}_1)^2 + \frac{735}{32} \hat{n} \cdot \vec{S}_1 \hat{n} \cdot \vec{S}_2 \hat{n} \cdot \vec{v}_2 \hat{n} \cdot \vec{v}_1 - \right. \right. \\ \left. \frac{105}{32} \hat{n} \cdot \vec{v}_2 \vec{S}_1 \cdot \vec{S}_2 \hat{n} \cdot \vec{v}_1 + \frac{15}{8} \hat{n} \cdot \vec{S}_2 \vec{S}_1 \cdot \vec{v}_1 \hat{n} \cdot \vec{v}_1 - \frac{105}{32} \hat{n} \cdot \vec{S}_2 \vec{S}_1 \cdot \vec{v}_2 \hat{n} \cdot \vec{v}_1 + \frac{15}{8} \hat{n} \cdot \vec{S}_1 \vec{S}_2 \cdot \vec{v}_1 \hat{n} \cdot \vec{v}_1 - \right. \\ \left. \frac{105}{32} \hat{n} \cdot \vec{S}_1 \vec{S}_2 \cdot \vec{v}_2 \hat{n} \cdot \vec{v}_1 - \frac{105}{16} \hat{n} \cdot \vec{S}_1 \hat{n} \cdot \vec{S}_2 (\hat{n} \cdot \vec{v}_2)^2 + \frac{15}{16} (\hat{n} \cdot \vec{v}_2)^2 \vec{S}_1 \cdot \vec{S}_2 - \frac{105}{32} \hat{n} \cdot \vec{S}_2 \hat{n} \cdot \vec{v}_2 \vec{S}_1 \cdot \vec{v}_1 + \right. \\ \left. \frac{15}{8} \hat{n} \cdot \vec{S}_2 \hat{n} \cdot \vec{v}_2 \vec{S}_1 \cdot \vec{v}_1 - \frac{105}{32} \hat{n} \cdot \vec{S}_2 \hat{n} \cdot \vec{v}_2 \vec{S}_1 \cdot \vec{v}_2 + \frac{15}{8} \hat{n} \cdot \vec{S}_1 \vec{S}_2 \cdot \vec{v}_1 \hat{n} \cdot \vec{v}_2 - \frac{105}{32} \hat{n} \cdot \vec{S}_1 \vec{S}_2 \cdot \vec{v}_2 \hat{n} \cdot \vec{v}_2 + \frac{15}{8} \hat{n} \cdot \vec{S}_1 \vec{S}_2 \cdot \vec{v}_2 \hat{n} \cdot \vec{v}_2 \right) \Bigg)$$

$$\left. \left. \left. \frac{15}{8} \hat{n} \cdot \vec{S}_2 \hat{n} \cdot \vec{v}_2 \vec{S}_1 \cdot \vec{v}_2 - \frac{105}{32} \hat{n} \cdot \vec{S}_1 \hat{n} \cdot \vec{v}_2 \vec{S}_2 \cdot \vec{v}_1 - \frac{3}{8} \vec{S}_1 \cdot \vec{v}_1 \vec{S}_2 \cdot \vec{v}_1 + \frac{21}{32} \vec{S}_1 \cdot \vec{v}_2 \vec{S}_2 \cdot \vec{v}_1 + \right. \right. \right. \\ \left. \left. \frac{15}{8} \hat{n} \cdot \vec{S}_1 \hat{n} \cdot \vec{v}_2 \vec{S}_2 \cdot \vec{v}_2 + \frac{21}{32} \vec{S}_1 \cdot \vec{v}_1 \vec{S}_2 \cdot \vec{v}_2 - \frac{3}{8} \vec{S}_1 \cdot \vec{v}_2 \vec{S}_2 \cdot \vec{v}_2 + \frac{15}{16} \hat{n} \cdot \vec{S}_1 \hat{n} \cdot \vec{S}_2 \vec{v}_1 \cdot \vec{v}_1 - \frac{3}{16} \vec{S}_1 \cdot \vec{S}_2 \vec{v}_1 \cdot \vec{v}_1 - \right. \right. \\ \left. \left. \frac{105}{32} \hat{n} \cdot \vec{S}_1 \hat{n} \cdot \vec{S}_2 \vec{v}_1 \cdot \vec{v}_2 + \frac{21}{32} \vec{S}_1 \cdot \vec{S}_2 \vec{v}_1 \cdot \vec{v}_2 + \frac{15}{16} \hat{n} \cdot \vec{S}_1 \hat{n} \cdot \vec{S}_2 \vec{v}_2 \cdot \vec{v}_2 - \frac{3}{16} \vec{S}_1 \cdot \vec{S}_2 \vec{v}_2 \cdot \vec{v}_2 \right) \right) \Bigg) \Bigg) m_1 m_2 \Bigg\}$$

{DiagS1S2[3, 9, 3],

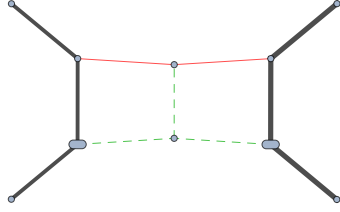

,

$$G^3 \left( \frac{1}{r^4} \left( -\frac{5}{2} \hat{n} \cdot \vec{a}_1 \hat{n} \cdot \vec{S}_1 \hat{n} \cdot \vec{S}_2 + \frac{5}{2} \hat{n} \cdot \vec{a}_2 \hat{n} \cdot \vec{S}_1 \hat{n} \cdot \vec{S}_2 - \frac{5}{2} \hat{n} \cdot \vec{S}_1 \hat{n} \cdot \vec{v}_1 \hat{n} \cdot \vec{S}_2 - 7 \hat{n} \cdot \vec{S}_1 \hat{n} \cdot \vec{v}_2 \hat{n} \cdot \vec{S}_2 - \right. \right. \\ \left. \left. \frac{1}{\vec{S}_1 \cdot \vec{v}_2} \hat{n} \cdot \vec{S}_2 + \vec{S}_1 \cdot \vec{a}_2 \hat{n} \cdot \vec{S}_2 + 7 \hat{n} \cdot \vec{S}_2 \hat{n} \cdot \vec{S}_1 \hat{n} \cdot \vec{v}_1 + \frac{5}{2} \hat{n} \cdot \vec{S}_2 \hat{n} \cdot \vec{S}_1 \hat{n} \cdot \vec{v}_2 + \frac{3}{2} \hat{n} \cdot \vec{v}_1 \vec{S}_1 \cdot \vec{S}_2 + \right. \right. \\ \left. \left. \frac{5}{2} \hat{n} \cdot \vec{v}_2 \vec{S}_1 \cdot \vec{S}_2 + \hat{n} \cdot \vec{S}_1 \vec{S}_2 \cdot \vec{v}_1 - \frac{5}{2} \hat{n} \cdot \vec{v}_1 \vec{S}_1 \cdot \vec{S}_2 - \frac{3}{2} \hat{n} \cdot \vec{v}_2 \vec{S}_1 \cdot \vec{S}_2 + \frac{3}{2} \hat{n} \cdot \vec{a}_1 \vec{S}_1 \cdot \vec{S}_2 - \right. \right. \\ \left. \left. \frac{3}{2} \hat{n} \cdot \vec{a}_2 \vec{S}_1 \cdot \vec{S}_2 - \frac{1}{2} \hat{n} \cdot \vec{S}_2 \vec{S}_1 \cdot \vec{v}_1 + \hat{n} \cdot \vec{S}_2 \vec{S}_1 \cdot \vec{v}_2 - \hat{n} \cdot \vec{S}_1 \vec{S}_2 \cdot \vec{a}_1 - \hat{n} \cdot \vec{S}_1 \vec{S}_2 \cdot \vec{v}_1 + \frac{1}{2} \hat{n} \cdot \vec{S}_1 \vec{S}_2 \cdot \vec{v}_2 \right) + \frac{1}{r^5} \right. \\ \left( \frac{93}{2} \hat{n} \cdot \vec{S}_1 \hat{n} \cdot \vec{S}_2 (\hat{n} \cdot \vec{v}_1)^2 - \frac{27}{2} \vec{S}_1 \cdot \vec{S}_2 (\hat{n} \cdot \vec{v}_1)^2 + \frac{307}{4} \hat{n} \cdot \vec{S}_1 \hat{n} \cdot \vec{S}_2 \hat{n} \cdot \vec{v}_2 \hat{n} \cdot \vec{v}_1 - \frac{57}{4} \hat{n} \cdot \vec{v}_2 \vec{S}_1 \cdot \vec{S}_2 \hat{n} \cdot \vec{v}_1 - \right. \\ \left. \frac{21}{2} \hat{n} \cdot \vec{S}_2 \vec{S}_1 \cdot \vec{v}_1 \hat{n} \cdot \vec{v}_1 - \frac{25}{4} \hat{n} \cdot \vec{S}_2 \vec{S}_1 \cdot \vec{v}_2 \hat{n} \cdot \vec{v}_1 - \frac{9}{2} \hat{n} \cdot \vec{S}_1 \vec{S}_2 \cdot \vec{v}_1 \hat{n} \cdot \vec{v}_1 - \frac{49}{4} \hat{n} \cdot \vec{S}_1 \vec{S}_2 \cdot \vec{v}_2 \hat{n} \cdot \vec{v}_1 + \right. \\ \left. \frac{93}{2} \hat{n} \cdot \vec{S}_1 \hat{n} \cdot \vec{S}_2 (\hat{n} \cdot \vec{v}_2)^2 - \hat{n} \times \vec{S}_1 \cdot \vec{v}_1 \hat{n} \times \vec{S}_2 \cdot \vec{v}_1 + \frac{1}{2} \hat{n} \times \vec{S}_1 \cdot \vec{v}_2 \hat{n} \times \vec{S}_2 \cdot \vec{v}_1 + \frac{11}{2} \hat{n} \times \vec{S}_1 \cdot \vec{v}_1 \hat{n} \times \vec{S}_2 \cdot \vec{v}_2 - \right. \\ \left. \hat{n} \times \vec{S}_1 \cdot \vec{v}_2 \hat{n} \times \vec{S}_2 \cdot \vec{v}_2 - \frac{27}{2} (\hat{n} \cdot \vec{v}_2)^2 \vec{S}_1 \cdot \vec{S}_2 - \frac{49}{4} \hat{n} \cdot \vec{S}_2 \hat{n} \cdot \vec{v}_2 \vec{S}_1 \cdot \vec{v}_1 - \frac{9}{2} \hat{n} \cdot \vec{S}_2 \hat{n} \cdot \vec{v}_2 \vec{S}_1 \cdot \vec{v}_2 - \frac{25}{4} \hat{n} \cdot \vec{S}_1 \hat{n} \cdot \vec{v}_2 \vec{S}_2 \cdot \vec{v}_1 - \right. \\ \left. \vec{S}_1 \cdot \vec{v}_1 \vec{S}_2 \cdot \vec{v}_1 - \frac{5}{4} \vec{S}_1 \cdot \vec{v}_2 \vec{S}_2 \cdot \vec{v}_1 - \frac{21}{2} \hat{n} \cdot \vec{S}_1 \hat{n} \cdot \vec{v}_2 \vec{S}_2 \cdot \vec{v}_2 + \frac{7}{4} \vec{S}_1 \cdot \vec{v}_1 \vec{S}_2 \cdot \vec{v}_2 - \vec{S}_1 \cdot \vec{v}_2 \vec{S}_2 \cdot \vec{v}_2 - \frac{11}{2} \hat{n} \cdot \vec{S}_1 \hat{n} \cdot \vec{S}_2 \vec{v}_1 \cdot \vec{v}_1 + \right. \\ \left. \frac{9}{2} \vec{S}_1 \cdot \vec{S}_2 \vec{v}_1 \cdot \vec{v}_1 - \frac{9}{4} \hat{n} \cdot \vec{S}_1 \hat{n} \cdot \vec{S}_2 \vec{v}_1 \cdot \vec{v}_2 + \frac{9}{4} \vec{S}_1 \cdot \vec{S}_2 \vec{v}_1 \cdot \vec{v}_2 - \frac{11}{2} \hat{n} \cdot \vec{S}_1 \hat{n} \cdot \vec{S}_2 \vec{v}_2 \cdot \vec{v}_2 + \frac{9}{2} \vec{S}_1 \cdot \vec{S}_2 \vec{v}_2 \cdot \vec{v}_2 \right) + \\ \pi^2 \left( \frac{1}{r^4} \left( -\frac{15}{32} \hat{n} \cdot \vec{S}_2 \hat{n} \cdot \vec{S}_1 \hat{n} \cdot \vec{v}_1 + \frac{3}{32} \vec{S}_1 \cdot \vec{S}_2 \hat{n} \cdot \vec{v}_1 + \frac{15}{32} \hat{n} \cdot \vec{S}_1 \hat{n} \cdot \vec{S}_2 \hat{n} \cdot \vec{v}_2 - \frac{3}{32} \hat{n} \cdot \vec{v}_2 \vec{S}_1 \cdot \vec{S}_2 - \right. \right. \\ \left. \left. \frac{3}{32} \hat{n} \cdot \vec{S}_2 \vec{S}_1 \cdot \vec{v}_2 + \frac{3}{32} \hat{n} \cdot \vec{S}_1 \vec{S}_2 \cdot \vec{v}_1 + \frac{3}{32} \hat{n} \cdot \vec{S}_2 \vec{S}_1 \cdot \vec{v}_1 - \frac{3}{32} \hat{n} \cdot \vec{S}_1 \vec{S}_2 \cdot \vec{v}_2 \right) + \frac{1}{r^5} \right. \\ \left( -\frac{105}{32} \hat{n} \cdot \vec{S}_1 \hat{n} \cdot \vec{S}_2 (\hat{n} \cdot \vec{v}_1)^2 + \frac{15}{32} \vec{S}_1 \cdot \vec{S}_2 (\hat{n} \cdot \vec{v}_1)^2 - \frac{105}{16} \hat{n} \cdot \vec{S}_1 \hat{n} \cdot \vec{S}_2 \hat{n} \cdot \vec{v}_2 \hat{n} \cdot \vec{v}_1 + \frac{15}{16} \hat{n} \cdot \vec{v}_2 \vec{S}_1 \cdot \vec{S}_2 \hat{n} \cdot \vec{v}_1 + \right. \\ \left. \frac{15}{16} \hat{n} \cdot \vec{S}_2 \vec{S}_1 \cdot \vec{v}_1 \hat{n} \cdot \vec{v}_1 + \frac{15}{16} \hat{n} \cdot \vec{S}_2 \vec{S}_1 \cdot \vec{v}_2 \hat{n} \cdot \vec{v}_1 + \frac{15}{16} \hat{n} \cdot \vec{S}_1 \vec{S}_2 \cdot \vec{v}_1 \hat{n} \cdot \vec{v}_1 + \frac{15}{16} \hat{n} \cdot \vec{S}_1 \vec{S}_2 \cdot \vec{v}_2 \hat{n} \cdot \vec{v}_1 - \right. \\ \left. \frac{105}{32} \hat{n} \cdot \vec{S}_1 \hat{n} \cdot \vec{S}_2 (\hat{n} \cdot \vec{v}_2)^2 + \frac{15}{32} (\hat{n} \cdot \vec{v}_2)^2 \vec{S}_1 \cdot \vec{S}_2 + \frac{15}{16} \hat{n} \cdot \vec{S}_2 \hat{n} \cdot \vec{v}_2 \vec{S}_1 \cdot \vec{v}_1 + \frac{15}{16} \hat{n} \cdot \vec{S}_2 \hat{n} \cdot \vec{v}_2 \vec{S}_1 \cdot \vec{v}_2 + \right. \\ \left. \frac{15}{16} \hat{n} \cdot \vec{S}_1 \hat{n} \cdot \vec{v}_2 \vec{S}_2 \cdot \vec{v}_1 - \frac{3}{16} \vec{S}_1 \cdot \vec{v}_1 \vec{S}_2 \cdot \vec{v}_1 - \frac{3}{16} \vec{S}_1 \cdot \vec{v}_2 \vec{S}_2 \cdot \vec{v}_1 + \frac{15}{16} \hat{n} \cdot \vec{S}_1 \hat{n} \cdot \vec{v}_2 \vec{S}_2 \cdot \vec{v}_2 - \right. \\ \left. \frac{3}{16} \vec{S}_1 \cdot \vec{v}_1 \vec{S}_2 \cdot \vec{v}_2 - \frac{3}{16} \vec{S}_1 \cdot \vec{v}_2 \vec{S}_2 \cdot \vec{v}_2 + \frac{15}{32} \hat{n} \cdot \vec{S}_1 \hat{n} \cdot \vec{S}_2 \vec{v}_1 \cdot \vec{v}_1 - \frac{3}{32} \vec{S}_1 \cdot \vec{S}_2 \vec{v}_1 \cdot \vec{v}_1 + \right. \\ \left. \frac{15}{16} \hat{n} \cdot \vec{S}_1 \hat{n} \cdot \vec{S}_2 \vec{v}_1 \cdot \vec{v}_2 - \frac{3}{16} \vec{S}_1 \cdot \vec{S}_2 \vec{v}_1 \cdot \vec{v}_2 + \frac{15}{32} \hat{n} \cdot \vec{S}_1 \hat{n} \cdot \vec{S}_2 \vec{v}_2 \cdot \vec{v}_2 - \frac{3}{32} \vec{S}_1 \cdot \vec{S}_2 \vec{v}_2 \cdot \vec{v}_2 \right) \Bigg) \Bigg) m_1 m_2 \Bigg\}$$



$\left\{ \text{DiagS1S2}[3, 9, 4], \right.$ 
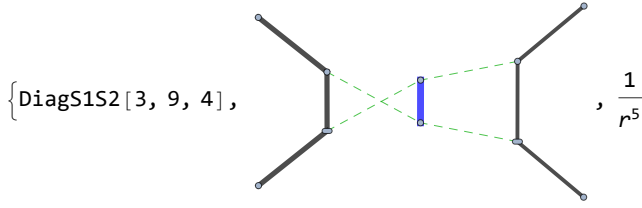
 $\left. , \frac{1}{r^5} \right\}$

$$G^3 m_1 m_2 \left( 75 \hat{n} \cdot \vec{S}_1 \cdot \vec{v}_2 \hat{n} \times \vec{S}_2 \cdot \vec{v}_1 - 41 \hat{n} \times \vec{S}_1 \cdot \vec{v}_1 \hat{n} \times \vec{S}_2 \cdot \vec{v}_2 + 66 \vec{S}_1 \cdot \vec{S}_2 \hat{n} \cdot \vec{v}_1 \hat{n} \cdot \vec{v}_2 - \right. \\ \left. 63 \hat{n} \cdot \vec{S}_2 \hat{n} \cdot \vec{v}_2 \vec{S}_1 \cdot \vec{v}_1 + 21 \hat{n} \cdot \vec{S}_2 \hat{n} \cdot \vec{v}_1 \vec{S}_1 \cdot \vec{v}_2 + 21 \hat{n} \cdot \vec{S}_1 \hat{n} \cdot \vec{v}_2 \vec{S}_2 \cdot \vec{v}_1 - 63 \hat{n} \cdot \vec{S}_1 \hat{n} \cdot \vec{v}_1 \vec{S}_2 \cdot \vec{v}_2 + \right. \\ \left. 10 \vec{v}_1 \cdot \vec{v}_2 \hat{n} \cdot \vec{S}_1 \hat{n} \cdot \vec{S}_2 - 9 \vec{S}_1 \cdot \vec{v}_2 \vec{S}_2 \cdot \vec{v}_1 + 91 \vec{S}_1 \cdot \vec{v}_1 \vec{S}_2 \cdot \vec{v}_2 - 74 \vec{S}_1 \cdot \vec{S}_2 \vec{v}_1 \cdot \vec{v}_2 \right) \Big\}$$

$\left\{ \text{DiagS1S2}[3, 9, 5], \right.$ 
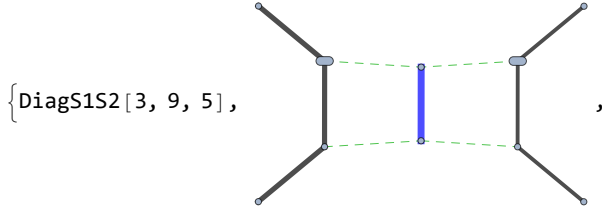
 $\left. , \right\}$

$$G^3 m_1 m_2 \left( \frac{1}{r^5} \left( 44 \hat{n} \times \vec{S}_1 \cdot \vec{v}_2 \hat{n} \times \vec{S}_2 \cdot \vec{v}_1 - 76 \hat{n} \times \vec{S}_1 \cdot \vec{v}_1 \hat{n} \times \vec{S}_2 \cdot \vec{v}_2 - 576 \hat{n} \cdot \vec{S}_1 \hat{n} \cdot \vec{S}_2 \hat{n} \cdot \vec{v}_1 \hat{n} \cdot \vec{v}_2 + \right. \right. \\ \left. 64 \vec{S}_1 \cdot \vec{S}_2 \hat{n} \cdot \vec{v}_1 \hat{n} \cdot \vec{v}_2 + 52 \hat{n} \cdot \vec{S}_2 \hat{n} \cdot \vec{v}_2 \vec{S}_1 \cdot \vec{v}_1 + 108 \hat{n} \cdot \vec{S}_2 \hat{n} \cdot \vec{v}_1 \vec{S}_1 \cdot \vec{v}_2 + 108 \hat{n} \cdot \vec{S}_1 \hat{n} \cdot \vec{v}_2 \vec{S}_2 \cdot \vec{v}_1 + \right. \\ \left. 52 \hat{n} \cdot \vec{S}_1 \hat{n} \cdot \vec{v}_1 \vec{S}_2 \cdot \vec{v}_2 + 264 \vec{v}_1 \cdot \vec{v}_2 \hat{n} \cdot \vec{S}_1 \hat{n} \cdot \vec{S}_2 - 60 \vec{S}_1 \cdot \vec{v}_2 \vec{S}_2 \cdot \vec{v}_1 + 20 \vec{S}_1 \cdot \vec{v}_1 \vec{S}_2 \cdot \vec{v}_2 - 32 \vec{S}_1 \cdot \vec{S}_2 \vec{v}_1 \cdot \vec{v}_2 \right) + \\ \left. \frac{1}{r^5} \pi^2 \left( \frac{945}{16} \hat{n} \cdot \vec{S}_1 \hat{n} \cdot \vec{S}_2 \hat{n} \cdot \vec{v}_1 \hat{n} \cdot \vec{v}_2 - \frac{135}{16} \vec{S}_1 \cdot \vec{S}_2 \hat{n} \cdot \vec{v}_1 \hat{n} \cdot \vec{v}_2 - \frac{135}{16} \hat{n} \cdot \vec{S}_2 \hat{n} \cdot \vec{v}_2 \vec{S}_1 \cdot \vec{v}_1 - \right. \right. \\ \left. \frac{135}{16} \hat{n} \cdot \vec{S}_1 \hat{n} \cdot \vec{v}_2 \vec{S}_2 \cdot \vec{v}_1 - \frac{135}{16} \hat{n} \cdot \vec{S}_2 \hat{n} \cdot \vec{v}_1 \vec{S}_1 \cdot \vec{v}_2 - \frac{135}{16} \hat{n} \cdot \vec{S}_1 \hat{n} \cdot \vec{v}_1 \vec{S}_2 \cdot \vec{v}_2 - \right. \\ \left. \frac{135}{16} \vec{v}_1 \cdot \vec{v}_2 \hat{n} \cdot \vec{S}_1 \hat{n} \cdot \vec{S}_2 + \frac{27}{16} \vec{S}_1 \cdot \vec{v}_2 \vec{S}_2 \cdot \vec{v}_1 + \frac{27}{16} \vec{S}_1 \cdot \vec{v}_1 \vec{S}_2 \cdot \vec{v}_2 + \frac{27}{16} \vec{S}_1 \cdot \vec{S}_2 \vec{v}_1 \cdot \vec{v}_2 \right) \Big\}$$

$\left\{ \text{DiagS1S2}[3, 9, 6], \right.$ 
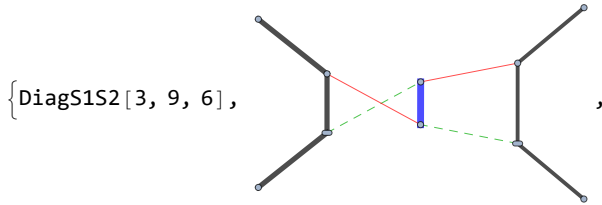
 $\left. , \right\}$

$$G^3 \left( \frac{22 \vec{S}_1 \cdot \vec{S}_2 - 42 \hat{n} \cdot \vec{S}_1 \hat{n} \cdot \vec{S}_2}{r^3} + \frac{1}{r^4} \left( 92 \hat{n} \cdot \vec{S}_2 \hat{n} \cdot \vec{S}_1 \hat{n} \cdot \vec{v}_1 + 110 \hat{n} \cdot \vec{S}_1 \hat{n} \cdot \vec{S}_2 \hat{n} \cdot \vec{v}_1 - \right. \right. \\ \left. 38 \vec{S}_1 \cdot \vec{S}_2 \hat{n} \cdot \vec{v}_1 - 30 \vec{S}_1 \cdot \vec{S}_2 \hat{n} \cdot \vec{v}_1 - 110 \hat{n} \cdot \vec{S}_2 \hat{n} \cdot \vec{S}_1 \hat{n} \cdot \vec{v}_2 - 92 \hat{n} \cdot \vec{S}_1 \hat{n} \cdot \vec{S}_2 \hat{n} \cdot \vec{v}_2 + 30 \hat{n} \cdot \vec{v}_2 \vec{S}_1 \cdot \vec{S}_2 - \right. \\ \left. 26 \hat{n} \cdot \vec{S}_2 \vec{S}_1 \cdot \vec{v}_1 + 26 \hat{n} \cdot \vec{S}_2 \vec{S}_1 \cdot \vec{v}_2 - 26 \hat{n} \cdot \vec{S}_1 \vec{S}_2 \cdot \vec{v}_1 + 26 \hat{n} \cdot \vec{S}_1 \vec{S}_2 \cdot \vec{v}_2 + 38 \hat{n} \cdot \vec{v}_2 \vec{S}_1 \cdot \vec{S}_2 - \right. \\ \left. 12 \hat{n} \cdot \vec{S}_2 \vec{S}_1 \cdot \vec{v}_1 + 10 \hat{n} \cdot \vec{S}_2 \vec{S}_1 \cdot \vec{v}_2 - 10 \hat{n} \cdot \vec{S}_1 \vec{S}_2 \cdot \vec{v}_1 + 12 \hat{n} \cdot \vec{S}_1 \vec{S}_2 \cdot \vec{v}_2 \right) + \frac{1}{r^5} \\ \left( -230 \hat{n} \cdot \vec{S}_1 \hat{n} \cdot \vec{S}_2 (\hat{n} \cdot \vec{v}_1)^2 + 30 \vec{S}_1 \cdot \vec{S}_2 (\hat{n} \cdot \vec{v}_1)^2 + 429 \hat{n} \cdot \vec{S}_1 \hat{n} \cdot \vec{S}_2 \hat{n} \cdot \vec{v}_2 \hat{n} \cdot \vec{v}_1 - 75 \hat{n} \cdot \vec{v}_2 \vec{S}_1 \cdot \vec{S}_2 \hat{n} \cdot \vec{v}_1 + \right. \\ \left. 72 \hat{n} \cdot \vec{S}_2 \vec{S}_1 \cdot \vec{v}_1 \hat{n} \cdot \vec{v}_1 - 79 \hat{n} \cdot \vec{S}_2 \vec{S}_1 \cdot \vec{v}_2 \hat{n} \cdot \vec{v}_1 + 76 \hat{n} \cdot \vec{S}_1 \vec{S}_2 \cdot \vec{v}_1 \hat{n} \cdot \vec{v}_1 - 55 \hat{n} \cdot \vec{S}_1 \vec{S}_2 \cdot \vec{v}_2 \hat{n} \cdot \vec{v}_1 - \right. \\ \left. 230 \hat{n} \cdot \vec{S}_1 \hat{n} \cdot \vec{S}_2 (\hat{n} \cdot \vec{v}_2)^2 + 12 \hat{n} \times \vec{S}_1 \cdot \vec{v}_1 \hat{n} \times \vec{S}_2 \cdot \vec{v}_1 - 12 \hat{n} \times \vec{S}_1 \cdot \vec{v}_2 \hat{n} \times \vec{S}_2 \cdot \vec{v}_1 - \right. \\ \left. 32 \hat{n} \times \vec{S}_1 \cdot \vec{v}_1 \hat{n} \times \vec{S}_2 \cdot \vec{v}_2 + 12 \hat{n} \times \vec{S}_1 \cdot \vec{v}_2 \hat{n} \times \vec{S}_2 \cdot \vec{v}_2 + 30 (\hat{n} \cdot \vec{v}_2)^2 \vec{S}_1 \cdot \vec{S}_2 - 55 \hat{n} \cdot \vec{S}_2 \hat{n} \cdot \vec{v}_2 \vec{S}_1 \cdot \vec{v}_1 + \right. \\ \left. 76 \hat{n} \cdot \vec{S}_2 \hat{n} \cdot \vec{v}_2 \vec{S}_1 \cdot \vec{v}_2 - 79 \hat{n} \cdot \vec{S}_1 \hat{n} \cdot \vec{v}_2 \vec{S}_2 \cdot \vec{v}_1 - 20 \vec{S}_1 \cdot \vec{v}_1 \vec{S}_2 \cdot \vec{v}_1 + 23 \vec{S}_1 \cdot \vec{v}_2 \vec{S}_2 \cdot \vec{v}_1 + \right. \\ \left. 72 \hat{n} \cdot \vec{S}_1 \hat{n} \cdot \vec{v}_2 \vec{S}_2 \cdot \vec{v}_2 + 11 \vec{S}_1 \cdot \vec{v}_1 \vec{S}_2 \cdot \vec{v}_2 - 20 \vec{S}_1 \cdot \vec{v}_2 \vec{S}_2 \cdot \vec{v}_2 + 2 \hat{n} \cdot \vec{S}_1 \hat{n} \cdot \vec{S}_2 \vec{v}_1 \cdot \vec{v}_1 + 22 \vec{S}_1 \cdot \vec{S}_2 \vec{v}_1 \cdot \vec{v}_1 - \right. \\ \left. 35 \hat{n} \cdot \vec{S}_1 \hat{n} \cdot \vec{S}_2 \vec{v}_1 \cdot \vec{v}_2 - 13 \vec{S}_1 \cdot \vec{S}_2 \vec{v}_1 \cdot \vec{v}_2 + 2 \hat{n} \cdot \vec{S}_1 \hat{n} \cdot \vec{S}_2 \vec{v}_2 \cdot \vec{v}_2 + 22 \vec{S}_1 \cdot \vec{S}_2 \vec{v}_2 \cdot \vec{v}_2 \right) + \right.$$

$$\begin{aligned}
& \pi^2 \left( \frac{3 \hat{n} \cdot \vec{S}_1 \hat{n} \cdot \vec{S}_2 - \vec{S}_1 \cdot \vec{S}_2}{r^3} + \frac{1}{r^4} \left( -\frac{45}{8} \hat{n} \cdot \vec{S}_2 \hat{n} \cdot \vec{S}_1 \hat{n} \cdot \vec{v}_1 - \frac{15}{2} \hat{n} \cdot \vec{S}_1 \hat{n} \cdot \vec{S}_2 \hat{n} \cdot \vec{v}_1 + \frac{3}{2} \vec{S}_1 \cdot \vec{S}_2 \hat{n} \cdot \vec{v}_1 + \right. \right. \\
& \quad \frac{9}{8} \vec{S}_1 \cdot \vec{S}_2 \hat{n} \cdot \vec{v}_1 + \frac{15}{2} \hat{n} \cdot \vec{S}_2 \hat{n} \cdot \vec{S}_1 \hat{n} \cdot \vec{v}_2 + \frac{45}{8} \hat{n} \cdot \vec{S}_1 \hat{n} \cdot \vec{S}_2 \hat{n} \cdot \vec{v}_2 - \frac{9}{8} \hat{n} \cdot \vec{v}_2 \vec{S}_1 \cdot \vec{S}_2 + \frac{3}{2} \hat{n} \cdot \vec{S}_2 \vec{S}_1 \cdot \vec{v}_1 - \\
& \quad \frac{9}{8} \hat{n} \cdot \vec{S}_2 \vec{S}_1 \cdot \vec{v}_2 + \frac{9}{8} \hat{n} \cdot \vec{S}_1 \vec{S}_2 \cdot \vec{v}_1 - \frac{3}{2} \hat{n} \cdot \vec{S}_1 \vec{S}_2 \cdot \vec{v}_2 - \frac{3}{2} \hat{n} \cdot \vec{v}_2 \vec{S}_1 \cdot \vec{S}_2 + \frac{9}{8} \hat{n} \cdot \vec{S}_2 \vec{S}_1 \cdot \vec{v}_1 - \frac{3}{2} \hat{n} \cdot \vec{S}_2 \vec{S}_1 \cdot \vec{v}_2 + \\
& \quad \left. \frac{3}{2} \hat{n} \cdot \vec{S}_1 \vec{S}_2 \cdot \vec{v}_1 - \frac{9}{8} \hat{n} \cdot \vec{S}_1 \vec{S}_2 \cdot \vec{v}_2 \right) + \frac{1}{r^5} \left( \frac{105}{8} \hat{n} \cdot \vec{S}_1 \hat{n} \cdot \vec{S}_2 (\hat{n} \cdot \vec{v}_1)^2 - \frac{15}{8} \vec{S}_1 \cdot \vec{S}_2 (\hat{n} \cdot \vec{v}_1)^2 - \right. \\
& \quad \frac{105}{4} \hat{n} \cdot \vec{S}_1 \hat{n} \cdot \vec{S}_2 \hat{n} \cdot \vec{v}_2 \hat{n} \cdot \vec{v}_1 + \frac{15}{4} \hat{n} \cdot \vec{v}_2 \vec{S}_1 \cdot \vec{S}_2 \hat{n} \cdot \vec{v}_1 - \frac{15}{4} \hat{n} \cdot \vec{S}_2 \vec{S}_1 \cdot \vec{v}_1 \hat{n} \cdot \vec{v}_1 + \frac{15}{4} \hat{n} \cdot \vec{S}_2 \vec{S}_1 \cdot \vec{v}_2 \hat{n} \cdot \vec{v}_1 - \\
& \quad \frac{15}{4} \hat{n} \cdot \vec{S}_1 \vec{S}_2 \cdot \vec{v}_1 \hat{n} \cdot \vec{v}_1 + \frac{15}{4} \hat{n} \cdot \vec{S}_1 \vec{S}_2 \cdot \vec{v}_2 \hat{n} \cdot \vec{v}_1 + \frac{105}{8} \hat{n} \cdot \vec{S}_1 \hat{n} \cdot \vec{S}_2 (\hat{n} \cdot \vec{v}_2)^2 - \frac{15}{8} (\hat{n} \cdot \vec{v}_2)^2 \vec{S}_1 \cdot \vec{S}_2 + \\
& \quad \frac{15}{4} \hat{n} \cdot \vec{S}_2 \hat{n} \cdot \vec{v}_2 \vec{S}_1 \cdot \vec{v}_1 - \frac{15}{4} \hat{n} \cdot \vec{S}_2 \hat{n} \cdot \vec{v}_2 \vec{S}_1 \cdot \vec{v}_2 + \frac{15}{4} \hat{n} \cdot \vec{S}_1 \hat{n} \cdot \vec{v}_2 \vec{S}_2 \cdot \vec{v}_1 + \frac{3}{4} \vec{S}_1 \cdot \vec{v}_1 \vec{S}_2 \cdot \vec{v}_1 - \frac{3}{4} \vec{S}_1 \cdot \vec{v}_2 \vec{S}_2 \cdot \vec{v}_1 - \\
& \quad \frac{15}{4} \hat{n} \cdot \vec{S}_1 \hat{n} \cdot \vec{v}_2 \vec{S}_2 \cdot \vec{v}_2 - \frac{3}{4} \vec{S}_1 \cdot \vec{v}_1 \vec{S}_2 \cdot \vec{v}_2 + \frac{3}{4} \vec{S}_1 \cdot \vec{v}_2 \vec{S}_2 \cdot \vec{v}_2 - \frac{15}{8} \hat{n} \cdot \vec{S}_1 \hat{n} \cdot \vec{S}_2 \vec{v}_1 \cdot \vec{v}_1 + \frac{3}{8} \vec{S}_1 \cdot \vec{S}_2 \vec{v}_1 \cdot \vec{v}_1 + \\
& \quad \left. \left. \frac{15}{4} \hat{n} \cdot \vec{S}_1 \hat{n} \cdot \vec{S}_2 \vec{v}_1 \cdot \vec{v}_2 - \frac{3}{4} \vec{S}_1 \cdot \vec{S}_2 \vec{v}_1 \cdot \vec{v}_2 - \frac{15}{8} \hat{n} \cdot \vec{S}_1 \hat{n} \cdot \vec{S}_2 \vec{v}_2 \cdot \vec{v}_2 + \frac{3}{8} \vec{S}_1 \cdot \vec{S}_2 \vec{v}_2 \cdot \vec{v}_2 \right) \right) \Bigg\} m_1 m_2 \Bigg\}
\end{aligned}$$

$$\left\{ \text{DiagS1S2}[3, 9, 7], \right.$$
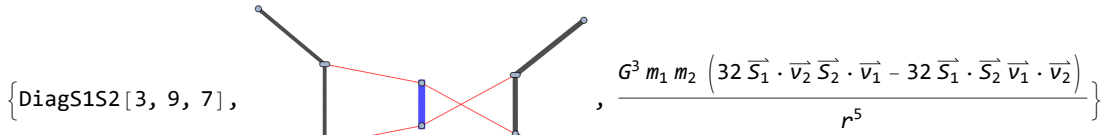

$$, \frac{G^3 m_1 m_2 (32 \vec{S}_1 \cdot \vec{v}_2 \vec{S}_2 \cdot \vec{v}_1 - 32 \vec{S}_1 \cdot \vec{S}_2 \vec{v}_1 \cdot \vec{v}_2)}{r^5} \Bigg\}$$

$$\left\{ \text{DiagS1S2}[3, 9, 8], \right.$$
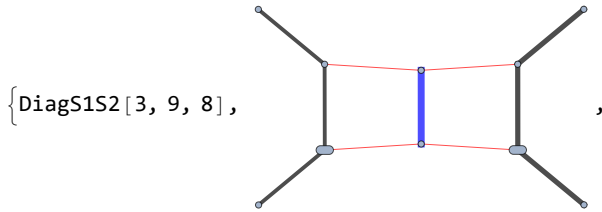

$$,$$

$$\frac{G^3 m_1 m_2 (-120 \hat{n} \times \vec{S}_1 \cdot \vec{v}_1 \hat{n} \times \vec{S}_2 \cdot \vec{v}_2 - 56 \vec{S}_1 \cdot \vec{v}_2 \vec{S}_2 \cdot \vec{v}_1 + 56 \vec{S}_1 \cdot \vec{S}_2 \vec{v}_1 \cdot \vec{v}_2)}{r^5} \Bigg\}$$

$$\left\{ \text{DiagS1S2}[3, 9, 9], \right.$$
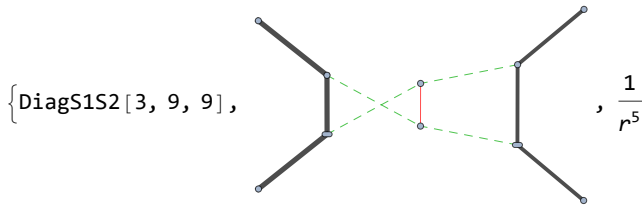

$$, \frac{1}{r^5} \Bigg\}$$

$$\begin{aligned}
& G^3 m_1 m_2 \left( -108 \hat{n} \times \vec{S}_1 \cdot \vec{v}_2 \hat{n} \times \vec{S}_2 \cdot \vec{v}_1 - 12 \hat{n} \times \vec{S}_1 \cdot \vec{v}_1 \hat{n} \times \vec{S}_2 \cdot \vec{v}_2 - 124 \hat{n} \cdot \vec{S}_1 \hat{n} \cdot \vec{S}_2 \hat{n} \cdot \vec{v}_1 \hat{n} \cdot \vec{v}_2 - 20 \vec{S}_1 \cdot \vec{S}_2 \hat{n} \cdot \vec{v}_1 \hat{n} \cdot \vec{v}_2 + \right. \\
& \quad \left. 72 \hat{n} \cdot \vec{S}_2 \hat{n} \cdot \vec{v}_2 \vec{S}_1 \cdot \vec{v}_1 + 72 \hat{n} \cdot \vec{S}_1 \hat{n} \cdot \vec{v}_1 \vec{S}_2 \cdot \vec{v}_2 + 12 \vec{v}_1 \cdot \vec{v}_2 \hat{n} \cdot \vec{S}_1 \hat{n} \cdot \vec{S}_2 - 48 \vec{S}_1 \cdot \vec{v}_1 \vec{S}_2 \cdot \vec{v}_2 + 36 \vec{S}_1 \cdot \vec{S}_2 \vec{v}_1 \cdot \vec{v}_2 \right) \Bigg\}
\end{aligned}$$

{DiagS1S2 [3, 9, 10],

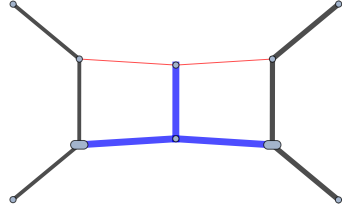

,

$$G^3 m_1 m_2 \left( \frac{1}{r^5} \left( -\frac{99}{2} \hat{n} \times \vec{S}_1 \cdot \vec{v}_2 \hat{n} \times \vec{S}_2 \cdot \vec{v}_1 + \frac{201}{2} \hat{n} \times \vec{S}_1 \cdot \vec{v}_1 \hat{n} \times \vec{S}_2 \cdot \vec{v}_2 + 41 \hat{n} \cdot \vec{S}_1 \hat{n} \cdot \vec{S}_2 \hat{n} \cdot \vec{v}_1 \hat{n} \cdot \vec{v}_2 + \right. \right. \\ \left. \left. 2 \vec{S}_1 \cdot \vec{S}_2 \hat{n} \cdot \vec{v}_1 \hat{n} \cdot \vec{v}_2 - \frac{3}{2} \hat{n} \cdot \vec{S}_2 \hat{n} \cdot \vec{v}_2 \vec{S}_1 \cdot \vec{v}_1 - \frac{37}{2} \hat{n} \cdot \vec{S}_2 \hat{n} \cdot \vec{v}_1 \vec{S}_1 \cdot \vec{v}_2 - \frac{37}{2} \hat{n} \cdot \vec{S}_1 \hat{n} \cdot \vec{v}_2 \vec{S}_2 \cdot \vec{v}_1 - \right. \right. \\ \left. \left. \frac{3}{2} \hat{n} \cdot \vec{S}_1 \hat{n} \cdot \vec{v}_1 \vec{S}_2 \cdot \vec{v}_2 + 48 \vec{v}_1 \cdot \vec{v}_2 \hat{n} \cdot \vec{S}_1 \hat{n} \cdot \vec{S}_2 + \frac{83}{2} \vec{S}_1 \cdot \vec{v}_2 \vec{S}_2 \cdot \vec{v}_1 - \frac{41}{2} \vec{S}_1 \cdot \vec{v}_1 \vec{S}_2 \cdot \vec{v}_2 - 28 \vec{S}_1 \cdot \vec{S}_2 \vec{v}_1 \cdot \vec{v}_2 \right) + \right. \\ \left. \frac{1}{r^5} \pi^2 \left( -\frac{315}{64} \hat{n} \cdot \vec{S}_1 \hat{n} \cdot \vec{S}_2 \hat{n} \cdot \vec{v}_1 \hat{n} \cdot \vec{v}_2 + \frac{45}{64} \vec{S}_1 \cdot \vec{S}_2 \hat{n} \cdot \vec{v}_1 \hat{n} \cdot \vec{v}_2 + \frac{45}{64} \hat{n} \cdot \vec{S}_2 \hat{n} \cdot \vec{v}_2 \vec{S}_1 \cdot \vec{v}_1 + \right. \right. \\ \left. \left. \frac{45}{64} \hat{n} \cdot \vec{S}_1 \hat{n} \cdot \vec{v}_2 \vec{S}_2 \cdot \vec{v}_1 + \frac{45}{64} \hat{n} \cdot \vec{S}_2 \hat{n} \cdot \vec{v}_1 \vec{S}_1 \cdot \vec{v}_2 + \frac{45}{64} \hat{n} \cdot \vec{S}_1 \hat{n} \cdot \vec{v}_1 \vec{S}_2 \cdot \vec{v}_2 + \right. \right. \\ \left. \left. \frac{45}{64} \vec{v}_1 \cdot \vec{v}_2 \hat{n} \cdot \vec{S}_1 \hat{n} \cdot \vec{S}_2 - \frac{9}{64} \vec{S}_1 \cdot \vec{v}_2 \vec{S}_2 \cdot \vec{v}_1 - \frac{9}{64} \vec{S}_1 \cdot \vec{v}_1 \vec{S}_2 \cdot \vec{v}_2 - \frac{9}{64} \vec{S}_1 \cdot \vec{S}_2 \vec{v}_1 \cdot \vec{v}_2 \right) \right) \Bigg\}$$

{DiagS1S2 [3, 9, 11],

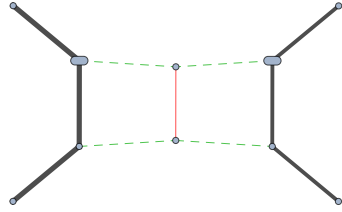

,  $\frac{1}{r^5}$

$$G^3 m_1 m_2 \left( -8 \hat{n} \cdot \vec{S}_2 \hat{n} \cdot \vec{v}_2 \vec{S}_1 \cdot \vec{v}_1 + 8 \hat{n} \cdot \vec{S}_2 \hat{n} \cdot \vec{v}_1 \vec{S}_1 \cdot \vec{v}_2 + 8 \hat{n} \cdot \vec{S}_1 \hat{n} \cdot \vec{v}_2 \vec{S}_2 \cdot \vec{v}_1 - \right. \\ \left. 8 \hat{n} \cdot \vec{S}_1 \hat{n} \cdot \vec{v}_1 \vec{S}_2 \cdot \vec{v}_2 + 64 \vec{v}_1 \cdot \vec{v}_2 \hat{n} \cdot \vec{S}_1 \hat{n} \cdot \vec{S}_2 - 32 \vec{S}_1 \cdot \vec{S}_2 \vec{v}_1 \cdot \vec{v}_2 \right) \Bigg\}$$

{DiagS1S2 [3, 9, 12],

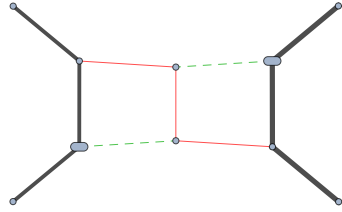

,

$$G^3 \left( \frac{\hat{n} \cdot \vec{S}_1 \hat{n} \cdot \vec{S}_2 - \vec{S}_1 \cdot \vec{S}_2}{r^3} + \frac{1}{r^4} \left( \frac{5}{2} \hat{n} \cdot \vec{a}_1 \hat{n} \cdot \vec{S}_1 \hat{n} \cdot \vec{S}_2 - \frac{5}{2} \hat{n} \cdot \vec{a}_2 \hat{n} \cdot \vec{S}_1 \hat{n} \cdot \vec{S}_2 - \frac{5}{2} \hat{n} \cdot \vec{S}_1 \hat{n} \cdot \vec{v}_1 \hat{n} \cdot \vec{S}_2 + \vec{S}_1 \cdot \vec{v}_1 \hat{n} \cdot \vec{S}_2 - \right. \right. \\ \left. \left. \frac{1}{\vec{S}_1 \cdot \vec{v}_2} \hat{n} \cdot \vec{S}_2 - \vec{S}_1 \cdot \vec{a}_1 \hat{n} \cdot \vec{S}_2 + \frac{5}{2} \hat{n} \cdot \vec{S}_2 \hat{n} \cdot \vec{S}_1 \hat{n} \cdot \vec{v}_2 + \frac{3}{2} \hat{n} \cdot \vec{v}_1 \vec{S}_1 \cdot \vec{S}_2 + \hat{n} \cdot \vec{S}_1 \vec{S}_2 \cdot \vec{v}_1 - \hat{n} \cdot \vec{S}_1 \vec{S}_2 \cdot \vec{v}_2 - \right. \right. \\ \left. \left. \frac{3}{2} \hat{n} \cdot \vec{v}_2 \vec{S}_1 \cdot \vec{S}_2 - \frac{3}{2} \hat{n} \cdot \vec{a}_1 \vec{S}_1 \cdot \vec{S}_2 + \frac{3}{2} \hat{n} \cdot \vec{a}_2 \vec{S}_1 \cdot \vec{S}_2 - \hat{n} \cdot \vec{S}_2 \vec{S}_1 \cdot \vec{v}_1 + \hat{n} \cdot \vec{S}_1 \vec{S}_2 \cdot \vec{a}_2 + \hat{n} \cdot \vec{S}_1 \vec{S}_2 \cdot \vec{v}_2 \right) + \frac{1}{r^5} \right. \\ \left( -\frac{9}{2} \hat{n} \cdot \vec{S}_1 \hat{n} \cdot \vec{S}_2 (\hat{n} \cdot \vec{v}_1)^2 + \frac{9}{2} \vec{S}_1 \cdot \vec{S}_2 (\hat{n} \cdot \vec{v}_1)^2 - \frac{15}{4} \hat{n} \cdot \vec{S}_1 \hat{n} \cdot \vec{S}_2 \hat{n} \cdot \vec{v}_2 \hat{n} \cdot \vec{v}_1 - \frac{5}{4} \hat{n} \cdot \vec{v}_2 \vec{S}_1 \cdot \vec{S}_2 \hat{n} \cdot \vec{v}_1 + \right. \\ \left. \frac{5}{2} \hat{n} \cdot \vec{S}_2 \vec{S}_1 \cdot \vec{v}_1 \hat{n} \cdot \vec{v}_1 - \frac{5}{2} \hat{n} \cdot \vec{S}_1 \vec{S}_2 \cdot \vec{v}_1 \hat{n} \cdot \vec{v}_1 + \frac{5}{2} \hat{n} \cdot \vec{S}_1 \vec{S}_2 \cdot \vec{v}_2 \hat{n} \cdot \vec{v}_1 - \frac{9}{2} \hat{n} \cdot \vec{S}_1 \hat{n} \cdot \vec{S}_2 (\hat{n} \cdot \vec{v}_2)^2 + \right. \\ \left. 2 \hat{n} \times \vec{S}_1 \cdot \vec{v}_1 \hat{n} \times \vec{S}_2 \cdot \vec{v}_1 - \frac{15}{4} \hat{n} \times \vec{S}_1 \cdot \vec{v}_2 \hat{n} \times \vec{S}_2 \cdot \vec{v}_1 - \frac{15}{4} \hat{n} \times \vec{S}_1 \cdot \vec{v}_1 \hat{n} \times \vec{S}_2 \cdot \vec{v}_2 + 2 \hat{n} \times \vec{S}_1 \cdot \vec{v}_2 \hat{n} \times \vec{S}_2 \cdot \vec{v}_2 + \right. \\ \left. \frac{9}{2} (\hat{n} \cdot \vec{v}_2)^2 \vec{S}_1 \cdot \vec{S}_2 + \frac{5}{2} \hat{n} \cdot \vec{S}_2 \hat{n} \cdot \vec{v}_2 \vec{S}_1 \cdot \vec{v}_1 - \frac{5}{2} \hat{n} \cdot \vec{S}_2 \hat{n} \cdot \vec{v}_2 \vec{S}_1 \cdot \vec{v}_2 + \vec{S}_1 \cdot \vec{v}_1 \vec{S}_2 \cdot \vec{v}_1 - \vec{S}_1 \cdot \vec{v}_2 \vec{S}_2 \cdot \vec{v}_1 + \right. \\ \left. \frac{5}{2} \vec{S}_1 \cdot \vec{v}_2 \vec{S}_2 \cdot \vec{v}_1 - \frac{5}{2} \vec{S}_1 \cdot \vec{v}_1 \vec{S}_2 \cdot \vec{v}_2 + \frac{5}{2} \vec{S}_1 \cdot \vec{v}_2 \vec{S}_2 \cdot \vec{v}_2 - \frac{5}{2} \vec{S}_1 \cdot \vec{v}_1 \vec{S}_2 \cdot \vec{v}_1 + \frac{5}{2} \vec{S}_1 \cdot \vec{v}_2 \vec{S}_2 \cdot \vec{v}_1 - \frac{5}{2} \vec{S}_1 \cdot \vec{v}_1 \vec{S}_2 \cdot \vec{v}_2 + \frac{5}{2} \vec{S}_1 \cdot \vec{v}_2 \vec{S}_2 \cdot \vec{v}_2 \right) \Bigg\}$$

$$\left. \begin{aligned} & \frac{5}{2} \hat{n} \cdot \vec{S}_1 \hat{n} \cdot \vec{v}_2 \vec{S}_2 \cdot \vec{v}_2 - 2 \vec{S}_1 \cdot \vec{v}_1 \vec{S}_2 \cdot \vec{v}_2 + \vec{S}_1 \cdot \vec{v}_2 \vec{S}_2 \cdot \vec{v}_2 + \frac{3}{2} \hat{n} \cdot \vec{S}_1 \hat{n} \cdot \vec{S}_2 \vec{v}_1 \cdot \vec{v}_1 - \frac{5}{2} \vec{S}_1 \cdot \vec{S}_2 \vec{v}_1 \cdot \vec{v}_1 - \\ & \frac{5}{4} \hat{n} \cdot \vec{S}_1 \hat{n} \cdot \vec{S}_2 \vec{v}_1 \cdot \vec{v}_2 + \frac{17}{4} \vec{S}_1 \cdot \vec{S}_2 \vec{v}_1 \cdot \vec{v}_2 + \frac{3}{2} \hat{n} \cdot \vec{S}_1 \hat{n} \cdot \vec{S}_2 \vec{v}_2 \cdot \vec{v}_2 - \frac{5}{2} \vec{S}_1 \cdot \vec{S}_2 \vec{v}_2 \cdot \vec{v}_2 \end{aligned} \right) m_1 m_2 \}$$

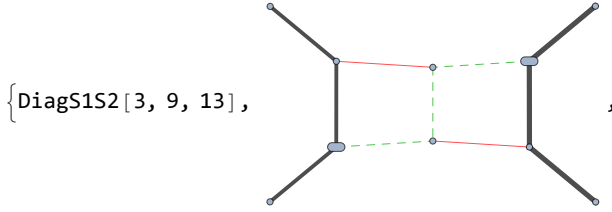

$$G^3 m_1 m_2 \left( \frac{1}{r^4} \left( 4 \vec{S}_1 \cdot \vec{a}_2 \hat{n} \cdot \vec{S}_2 + 4 \vec{S}_1 \cdot \vec{S}_2 \hat{n} \cdot \vec{a}_1 - 4 \vec{S}_1 \cdot \vec{S}_2 \hat{n} \cdot \vec{a}_2 - 4 \vec{S}_2 \cdot \vec{a}_1 \hat{n} \cdot \vec{S}_1 + 4 \vec{S}_1 \cdot \vec{S}_2 \hat{n} \cdot \vec{v}_1 - \right. \right. \\ \left. \left. 4 \vec{S}_1 \cdot \vec{S}_2 \hat{n} \cdot \vec{v}_2 + 4 \hat{n} \cdot \vec{S}_2 \vec{S}_1 \cdot \vec{v}_2 - 4 \hat{n} \cdot \vec{S}_1 \vec{S}_2 \cdot \vec{v}_1 \right) + \frac{1}{r^5} \left( 14 \hat{n} \times \vec{S}_1 \cdot \vec{v}_1 \hat{n} \times \vec{S}_2 \cdot \vec{v}_1 + 14 \hat{n} \times \vec{S}_1 \cdot \vec{v}_2 \hat{n} \times \vec{S}_2 \cdot \vec{v}_2 - \right. \right. \\ \left. \left. 2 \vec{S}_1 \cdot \vec{S}_2 (\hat{n} \cdot \vec{v}_1)^2 + 2 \hat{n} \cdot \vec{S}_1 \hat{n} \cdot \vec{v}_1 \vec{S}_2 \cdot \vec{v}_1 - 2 \vec{S}_1 \cdot \vec{S}_2 (\hat{n} \cdot \vec{v}_2)^2 + 2 \hat{n} \cdot \vec{S}_2 \hat{n} \cdot \vec{v}_2 \vec{S}_1 \cdot \vec{v}_2 - 18 \vec{v}_1 \cdot \vec{v}_1 \hat{n} \cdot \vec{S}_1 \hat{n} \cdot \vec{S}_2 - \right. \right. \\ \left. \left. 18 \vec{v}_2 \cdot \vec{v}_2 \hat{n} \cdot \vec{S}_1 \hat{n} \cdot \vec{S}_2 + 4 \vec{S}_1 \cdot \vec{v}_1 \vec{S}_2 \cdot \vec{v}_1 + 4 \vec{S}_1 \cdot \vec{v}_2 \vec{S}_2 \cdot \vec{v}_2 + 2 \vec{S}_1 \cdot \vec{S}_2 \vec{v}_1 \cdot \vec{v}_1 + 2 \vec{S}_1 \cdot \vec{S}_2 \vec{v}_2 \cdot \vec{v}_2 \right) \right) \}$$

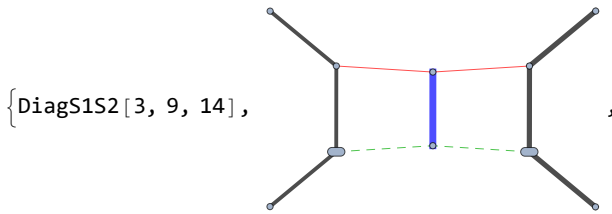

$$G^3 \left( \frac{15 \hat{n} \cdot \vec{S}_1 \hat{n} \cdot \vec{S}_2 - 7 \vec{S}_1 \cdot \vec{S}_2}{r^3} + \frac{1}{r^4} \left( -\frac{67}{2} \hat{n} \cdot \vec{S}_2 \hat{n} \cdot \vec{S}_1 \hat{n} \cdot \vec{v}_1 + 16 \vec{S}_1 \cdot \vec{S}_2 \hat{n} \cdot \vec{v}_1 + 10 \vec{S}_1 \cdot \vec{S}_2 \hat{n} \cdot \vec{v}_1 + \frac{67}{2} \hat{n} \cdot \vec{S}_1 \hat{n} \cdot \vec{S}_2 \hat{n} \cdot \vec{v}_2 - \right. \right. \\ \left. \left. 10 \hat{n} \cdot \vec{v}_2 \vec{S}_1 \cdot \vec{S}_2 - 7 \hat{n} \cdot \vec{S}_2 \vec{S}_1 \cdot \vec{v}_2 + 7 \hat{n} \cdot \vec{S}_1 \vec{S}_2 \cdot \vec{v}_1 - 16 \hat{n} \cdot \vec{v}_2 \vec{S}_1 \cdot \vec{S}_2 + 16 \hat{n} \cdot \vec{S}_2 \vec{S}_1 \cdot \vec{a}_2 + 16 \hat{n} \cdot \vec{a}_1 \vec{S}_1 \cdot \vec{S}_2 - \right. \right. \\ \left. \left. 16 \hat{n} \cdot \vec{a}_2 \vec{S}_1 \cdot \vec{S}_2 + \frac{11}{2} \hat{n} \cdot \vec{S}_2 \vec{S}_1 \cdot \vec{v}_1 + 16 \hat{n} \cdot \vec{S}_2 \vec{S}_1 \cdot \vec{v}_2 - 16 \hat{n} \cdot \vec{S}_1 \vec{S}_2 \cdot \vec{a}_1 - 16 \hat{n} \cdot \vec{S}_1 \vec{S}_2 \cdot \vec{v}_1 - \frac{11}{2} \hat{n} \cdot \vec{S}_1 \vec{S}_2 \cdot \vec{v}_2 \right) + \pi^2 \right. \\ \left. \left( \frac{\frac{3}{8} \vec{S}_1 \cdot \vec{S}_2 - \frac{9}{8} \hat{n} \cdot \vec{S}_1 \hat{n} \cdot \vec{S}_2}{r^3} + \frac{1}{r^4} \left( \frac{75}{32} \hat{n} \cdot \vec{S}_2 \hat{n} \cdot \vec{S}_1 \hat{n} \cdot \vec{v}_1 - \frac{15}{32} \vec{S}_1 \cdot \vec{S}_2 \hat{n} \cdot \vec{v}_1 - \frac{75}{32} \hat{n} \cdot \vec{S}_1 \hat{n} \cdot \vec{S}_2 \hat{n} \cdot \vec{v}_2 + \frac{15}{32} \hat{n} \cdot \vec{v}_2 \vec{S}_1 \cdot \vec{S}_2 + \right. \right. \right. \\ \left. \left. \frac{15}{32} \hat{n} \cdot \vec{S}_2 \vec{S}_1 \cdot \vec{v}_2 - \frac{15}{32} \hat{n} \cdot \vec{S}_1 \vec{S}_2 \cdot \vec{v}_1 - \frac{15}{32} \hat{n} \cdot \vec{S}_2 \vec{S}_1 \cdot \vec{v}_1 + \frac{15}{32} \hat{n} \cdot \vec{S}_1 \vec{S}_2 \cdot \vec{v}_2 \right) + \frac{1}{r^5} \left( \frac{735}{64} \hat{n} \cdot \vec{S}_1 \hat{n} \cdot \vec{S}_2 \hat{n} \cdot \vec{v}_1 \hat{n} \cdot \vec{v}_2 - \right. \right. \\ \left. \left. \frac{105}{64} \hat{n} \cdot \vec{v}_1 \vec{S}_1 \cdot \vec{S}_2 \hat{n} \cdot \vec{v}_2 - \frac{105}{64} \hat{n} \cdot \vec{S}_2 \vec{S}_1 \cdot \vec{v}_1 \hat{n} \cdot \vec{v}_2 - \frac{105}{64} \hat{n} \cdot \vec{S}_1 \vec{S}_2 \cdot \vec{v}_1 \hat{n} \cdot \vec{v}_2 - \frac{105}{64} \hat{n} \cdot \vec{S}_2 \hat{n} \cdot \vec{v}_1 \vec{S}_1 \cdot \vec{v}_2 + \right. \right. \\ \left. \left. \frac{21}{64} \vec{S}_1 \cdot \vec{v}_2 \vec{S}_2 \cdot \vec{v}_1 - \frac{105}{64} \hat{n} \cdot \vec{S}_1 \hat{n} \cdot \vec{v}_1 \vec{S}_2 \cdot \vec{v}_2 + \frac{21}{64} \vec{S}_1 \cdot \vec{v}_1 \vec{S}_2 \cdot \vec{v}_2 - \frac{105}{64} \hat{n} \cdot \vec{S}_1 \hat{n} \cdot \vec{S}_2 \vec{v}_1 \cdot \vec{v}_2 + \frac{21}{64} \vec{S}_1 \cdot \vec{S}_2 \vec{v}_1 \cdot \vec{v}_2 \right) \right) + \\ \left. \frac{1}{r^5} \left( -11 \vec{S}_1 \cdot \vec{S}_2 (\hat{n} \cdot \vec{v}_1)^2 - \frac{707}{4} \hat{n} \cdot \vec{S}_1 \hat{n} \cdot \vec{S}_2 \hat{n} \cdot \vec{v}_2 \hat{n} \cdot \vec{v}_1 + \frac{157}{4} \hat{n} \cdot \vec{v}_2 \vec{S}_1 \cdot \vec{S}_2 \hat{n} \cdot \vec{v}_1 + \frac{97}{4} \hat{n} \cdot \vec{S}_2 \vec{S}_1 \cdot \vec{v}_2 \hat{n} \cdot \vec{v}_1 + \right. \right. \\ \left. \left. 11 \hat{n} \cdot \vec{S}_1 \vec{S}_2 \cdot \vec{v}_1 \hat{n} \cdot \vec{v}_1 + \frac{77}{4} \hat{n} \cdot \vec{S}_1 \vec{S}_2 \cdot \vec{v}_2 \hat{n} \cdot \vec{v}_1 + 61 \hat{n} \times \vec{S}_1 \cdot \vec{v}_1 \hat{n} \times \vec{S}_2 \cdot \vec{v}_1 - 3 \hat{n} \times \vec{S}_1 \cdot \vec{v}_2 \hat{n} \times \vec{S}_2 \cdot \vec{v}_1 - \right. \right. \\ \left. \left. 8 \hat{n} \times \vec{S}_1 \cdot \vec{v}_1 \hat{n} \times \vec{S}_2 \cdot \vec{v}_2 + 61 \hat{n} \times \vec{S}_1 \cdot \vec{v}_2 \hat{n} \times \vec{S}_2 \cdot \vec{v}_2 - 11 (\hat{n} \cdot \vec{v}_2)^2 \vec{S}_1 \cdot \vec{S}_2 + \frac{77}{4} \hat{n} \cdot \vec{S}_2 \hat{n} \cdot \vec{v}_2 \vec{S}_1 \cdot \vec{v}_1 + \right. \right. \end{aligned} \right)$$

$$\left. \begin{aligned} & 11 \hat{n} \cdot \vec{S}_2 \hat{n} \cdot \vec{v}_2 \vec{S}_1 \cdot \vec{v}_2 + \frac{97}{4} \hat{n} \cdot \vec{S}_1 \hat{n} \cdot \vec{v}_2 \vec{S}_2 \cdot \vec{v}_1 + 20 \vec{S}_1 \cdot \vec{v}_1 \vec{S}_2 \cdot \vec{v}_1 - \frac{25}{4} \vec{S}_1 \cdot \vec{v}_2 \vec{S}_2 \cdot \vec{v}_1 - \\ & \frac{13}{4} \vec{S}_1 \cdot \vec{v}_1 \vec{S}_2 \cdot \vec{v}_2 + 20 \vec{S}_1 \cdot \vec{v}_2 \vec{S}_2 \cdot \vec{v}_2 - 75 \hat{n} \cdot \vec{S}_1 \hat{n} \cdot \vec{S}_2 \vec{v}_1 \cdot \vec{v}_1 - 5 \vec{S}_1 \cdot \vec{S}_2 \vec{v}_1 \cdot \vec{v}_1 + \\ & \frac{125}{4} \hat{n} \cdot \vec{S}_1 \hat{n} \cdot \vec{S}_2 \vec{v}_1 \cdot \vec{v}_2 - \frac{37}{4} \vec{S}_1 \cdot \vec{S}_2 \vec{v}_1 \cdot \vec{v}_2 - 75 \hat{n} \cdot \vec{S}_1 \hat{n} \cdot \vec{S}_2 \vec{v}_2 \cdot \vec{v}_2 - 5 \vec{S}_1 \cdot \vec{S}_2 \vec{v}_2 \cdot \vec{v}_2 \end{aligned} \right) m_1 m_2 \}$$

{DiagS1S2[3, 9, 15],

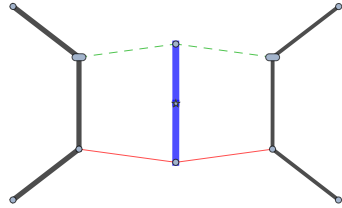

,

$$\begin{aligned} G^3 \left( \frac{1}{r^4} \left( -\frac{5}{2} \hat{n} \cdot \vec{S}_2 \hat{n} \cdot \vec{S}_1 \hat{n} \cdot \vec{v}_1 - \frac{5}{2} \hat{n} \cdot \vec{S}_1 \hat{n} \cdot \vec{S}_2 \hat{n} \cdot \vec{v}_1 + \frac{1}{2} \vec{S}_1 \cdot \vec{S}_2 \hat{n} \cdot \vec{v}_1 + \frac{1}{2} \vec{S}_1 \cdot \vec{S}_2 \hat{n} \cdot \vec{v}_1 + \frac{5}{2} \hat{n} \cdot \vec{S}_2 \hat{n} \cdot \vec{S}_1 \hat{n} \cdot \vec{v}_2 + \right. \right. \\ \left. \frac{5}{2} \hat{n} \cdot \vec{S}_1 \hat{n} \cdot \vec{S}_2 \hat{n} \cdot \vec{v}_2 - \frac{1}{2} \hat{n} \cdot \vec{v}_2 \vec{S}_1 \cdot \vec{S}_2 - \frac{1}{2} \hat{n} \cdot \vec{S}_2 \vec{S}_1 \cdot \vec{v}_1 + \frac{1}{2} \hat{n} \cdot \vec{S}_2 \vec{S}_1 \cdot \vec{v}_2 - \frac{1}{2} \hat{n} \cdot \vec{S}_1 \vec{S}_2 \cdot \vec{v}_1 + \right. \\ \left. \frac{1}{2} \hat{n} \cdot \vec{S}_1 \vec{S}_2 \cdot \vec{v}_2 - \frac{1}{2} \hat{n} \cdot \vec{v}_2 \vec{S}_1 \cdot \vec{S}_2 - \frac{1}{2} \hat{n} \cdot \vec{S}_2 \vec{S}_1 \cdot \vec{v}_1 + \frac{1}{2} \hat{n} \cdot \vec{S}_2 \vec{S}_1 \cdot \vec{v}_2 - \frac{1}{2} \hat{n} \cdot \vec{S}_1 \vec{S}_2 \cdot \vec{v}_1 + \frac{1}{2} \hat{n} \cdot \vec{S}_1 \vec{S}_2 \cdot \vec{v}_2 \right) + \\ \frac{1}{r^5} \pi^2 \left( -\frac{105}{128} \hat{n} \cdot \vec{S}_1 \hat{n} \cdot \vec{S}_2 (\hat{n} \cdot \vec{v}_1)^2 + \frac{15}{128} \vec{S}_1 \cdot \vec{S}_2 (\hat{n} \cdot \vec{v}_1)^2 - \frac{315}{32} \hat{n} \cdot \vec{S}_1 \hat{n} \cdot \vec{S}_2 \hat{n} \cdot \vec{v}_2 \hat{n} \cdot \vec{v}_1 + \right. \\ \frac{45}{32} \hat{n} \cdot \vec{v}_2 \vec{S}_1 \cdot \vec{S}_2 \hat{n} \cdot \vec{v}_1 + \frac{15}{64} \hat{n} \cdot \vec{S}_2 \vec{S}_1 \cdot \vec{v}_1 \hat{n} \cdot \vec{v}_1 + \frac{45}{32} \hat{n} \cdot \vec{S}_2 \vec{S}_1 \cdot \vec{v}_2 \hat{n} \cdot \vec{v}_1 + \frac{15}{64} \hat{n} \cdot \vec{S}_1 \vec{S}_2 \cdot \vec{v}_1 \hat{n} \cdot \vec{v}_1 + \\ \frac{45}{32} \hat{n} \cdot \vec{S}_1 \vec{S}_2 \cdot \vec{v}_2 \hat{n} \cdot \vec{v}_1 - \frac{105}{128} \hat{n} \cdot \vec{S}_1 \hat{n} \cdot \vec{S}_2 (\hat{n} \cdot \vec{v}_2)^2 + \frac{15}{128} (\hat{n} \cdot \vec{v}_2)^2 \vec{S}_1 \cdot \vec{S}_2 + \frac{45}{32} \hat{n} \cdot \vec{S}_2 \hat{n} \cdot \vec{v}_2 \vec{S}_1 \cdot \vec{v}_1 + \\ \frac{15}{64} \hat{n} \cdot \vec{S}_2 \hat{n} \cdot \vec{v}_2 \vec{S}_1 \cdot \vec{v}_2 + \frac{45}{32} \hat{n} \cdot \vec{S}_1 \hat{n} \cdot \vec{v}_2 \vec{S}_2 \cdot \vec{v}_1 - \frac{3}{64} \vec{S}_1 \cdot \vec{v}_1 \vec{S}_2 \cdot \vec{v}_1 - \frac{9}{32} \vec{S}_1 \cdot \vec{v}_2 \vec{S}_2 \cdot \vec{v}_1 + \\ \frac{15}{64} \hat{n} \cdot \vec{S}_1 \hat{n} \cdot \vec{v}_2 \vec{S}_2 \cdot \vec{v}_2 - \frac{9}{32} \vec{S}_1 \cdot \vec{v}_1 \vec{S}_2 \cdot \vec{v}_2 - \frac{3}{64} \vec{S}_1 \cdot \vec{v}_2 \vec{S}_2 \cdot \vec{v}_2 + \frac{15}{128} \hat{n} \cdot \vec{S}_1 \hat{n} \cdot \vec{S}_2 \vec{v}_1 \cdot \vec{v}_1 - \frac{3}{128} \vec{S}_1 \cdot \vec{S}_2 \vec{v}_1 \cdot \vec{v}_1 + \\ \frac{45}{32} \hat{n} \cdot \vec{S}_1 \hat{n} \cdot \vec{S}_2 \vec{v}_1 \cdot \vec{v}_2 - \frac{9}{32} \vec{S}_1 \cdot \vec{S}_2 \vec{v}_1 \cdot \vec{v}_2 + \frac{15}{128} \hat{n} \cdot \vec{S}_1 \hat{n} \cdot \vec{S}_2 \vec{v}_2 \cdot \vec{v}_2 - \frac{3}{128} \vec{S}_1 \cdot \vec{S}_2 \vec{v}_2 \cdot \vec{v}_2 \left. \right) + \frac{1}{r^5} \\ \left( \frac{119}{24} \hat{n} \cdot \vec{S}_1 \hat{n} \cdot \vec{S}_2 (\hat{n} \cdot \vec{v}_1)^2 - \frac{89}{24} \vec{S}_1 \cdot \vec{S}_2 (\hat{n} \cdot \vec{v}_1)^2 + \frac{203}{2} \hat{n} \cdot \vec{S}_1 \hat{n} \cdot \vec{S}_2 \hat{n} \cdot \vec{v}_2 \hat{n} \cdot \vec{v}_1 - \frac{13}{2} \hat{n} \cdot \vec{v}_2 \vec{S}_1 \cdot \vec{S}_2 \hat{n} \cdot \vec{v}_1 + \right. \\ \frac{43}{12} \hat{n} \cdot \vec{S}_2 \vec{S}_1 \cdot \vec{v}_1 \hat{n} \cdot \vec{v}_1 - \frac{27}{2} \hat{n} \cdot \vec{S}_2 \vec{S}_1 \cdot \vec{v}_2 \hat{n} \cdot \vec{v}_1 - \frac{41}{12} \hat{n} \cdot \vec{S}_1 \vec{S}_2 \cdot \vec{v}_1 \hat{n} \cdot \vec{v}_1 - \frac{39}{2} \hat{n} \cdot \vec{S}_1 \vec{S}_2 \cdot \vec{v}_2 \hat{n} \cdot \vec{v}_1 + \\ \frac{119}{24} \hat{n} \cdot \vec{S}_1 \hat{n} \cdot \vec{S}_2 (\hat{n} \cdot \vec{v}_2)^2 - 5 \hat{n} \times \vec{S}_1 \cdot \vec{v}_1 \hat{n} \times \vec{S}_2 \cdot \vec{v}_1 + 14 \hat{n} \times \vec{S}_1 \cdot \vec{v}_2 \hat{n} \times \vec{S}_2 \cdot \vec{v}_1 - 4 \hat{n} \times \vec{S}_1 \cdot \vec{v}_1 \hat{n} \times \vec{S}_2 \cdot \vec{v}_2 - \\ 5 \hat{n} \times \vec{S}_1 \cdot \vec{v}_2 \hat{n} \times \vec{S}_2 \cdot \vec{v}_2 - \frac{89}{24} (\hat{n} \cdot \vec{v}_2)^2 \vec{S}_1 \cdot \vec{S}_2 - \frac{39}{2} \hat{n} \cdot \vec{S}_2 \hat{n} \cdot \vec{v}_2 \vec{S}_1 \cdot \vec{v}_1 - \frac{41}{12} \hat{n} \cdot \vec{S}_2 \hat{n} \cdot \vec{v}_2 \vec{S}_1 \cdot \vec{v}_2 - \\ \frac{27}{2} \hat{n} \cdot \vec{S}_1 \hat{n} \cdot \vec{v}_2 \vec{S}_2 \cdot \vec{v}_1 - \frac{35}{12} \vec{S}_1 \cdot \vec{v}_1 \vec{S}_2 \cdot \vec{v}_1 + \frac{1}{2} \vec{S}_1 \cdot \vec{v}_2 \vec{S}_2 \cdot \vec{v}_1 + \frac{43}{12} \hat{n} \cdot \vec{S}_1 \hat{n} \cdot \vec{v}_2 \vec{S}_2 \cdot \vec{v}_2 + \\ \frac{25}{2} \vec{S}_1 \cdot \vec{v}_1 \vec{S}_2 \cdot \vec{v}_2 - \frac{35}{12} \vec{S}_1 \cdot \vec{v}_2 \vec{S}_2 \cdot \vec{v}_2 + \frac{79}{24} \hat{n} \cdot \vec{S}_1 \hat{n} \cdot \vec{S}_2 \vec{v}_1 \cdot \vec{v}_1 + \frac{61}{24} \vec{S}_1 \cdot \vec{S}_2 \vec{v}_1 \cdot \vec{v}_1 - \\ \left. \frac{77}{2} \hat{n} \cdot \vec{S}_1 \hat{n} \cdot \vec{S}_2 \vec{v}_1 \cdot \vec{v}_2 + \frac{1}{2} \vec{S}_1 \cdot \vec{S}_2 \vec{v}_1 \cdot \vec{v}_2 + \frac{79}{24} \hat{n} \cdot \vec{S}_1 \hat{n} \cdot \vec{S}_2 \vec{v}_2 \cdot \vec{v}_2 + \frac{61}{24} \vec{S}_1 \cdot \vec{S}_2 \vec{v}_2 \cdot \vec{v}_2 \right) m_1 m_2 \} \end{aligned}$$

{DiagS1S2[3, 9, 16],

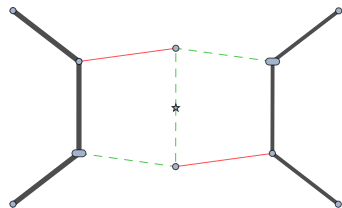

,

$$\begin{aligned}
& G^3 \left( \frac{4 \vec{S}_1 \cdot \vec{S}_2 - 32 \hat{n} \cdot \vec{S}_1 \hat{n} \cdot \vec{S}_2}{r^3} + \frac{1}{r^4} \left( 91 \hat{n} \cdot \vec{S}_2 \hat{n} \cdot \vec{S}_1 \hat{n} \cdot \vec{v}_1 + 69 \hat{n} \cdot \vec{S}_1 \hat{n} \cdot \vec{S}_2 \hat{n} \cdot \vec{v}_1 - 9 \vec{S}_1 \cdot \vec{S}_2 \hat{n} \cdot \vec{v}_1 - 3 \vec{S}_1 \cdot \vec{S}_2 \hat{n} \cdot \vec{v}_1 - \right. \right. \\
& 69 \hat{n} \cdot \vec{S}_2 \hat{n} \cdot \vec{S}_1 \hat{n} \cdot \vec{v}_2 - 91 \hat{n} \cdot \vec{S}_1 \hat{n} \cdot \vec{S}_2 \hat{n} \cdot \vec{v}_2 + 3 \hat{n} \cdot \vec{v}_2 \vec{S}_1 \cdot \vec{S}_2 - 9 \hat{n} \cdot \vec{S}_2 \vec{S}_1 \cdot \vec{v}_1 + 19 \hat{n} \cdot \vec{S}_2 \vec{S}_1 \cdot \vec{v}_2 - 19 \hat{n} \cdot \vec{S}_1 \vec{S}_2 \cdot \vec{v}_1 + \\
& 9 \hat{n} \cdot \vec{S}_1 \vec{S}_2 \cdot \vec{v}_2 + 9 \hat{n} \cdot \vec{v}_2 \vec{S}_1 \cdot \vec{S}_2 - 23 \hat{n} \cdot \vec{S}_2 \vec{S}_1 \cdot \vec{v}_1 + 13 \hat{n} \cdot \vec{S}_2 \vec{S}_1 \cdot \vec{v}_2 - 13 \hat{n} \cdot \vec{S}_1 \vec{S}_2 \cdot \vec{v}_1 + 23 \hat{n} \cdot \vec{S}_1 \vec{S}_2 \cdot \vec{v}_2 \Big) + \\
& \pi^2 \left( \frac{\frac{1}{4} \vec{S}_1 \cdot \vec{S}_2 - \frac{3}{4} \hat{n} \cdot \vec{S}_1 \hat{n} \cdot \vec{S}_2}{r^3} + \frac{1}{r^4} \left( \frac{75}{16} \hat{n} \cdot \vec{S}_2 \hat{n} \cdot \vec{S}_1 \hat{n} \cdot \vec{v}_1 - \frac{15}{16} \hat{n} \cdot \vec{S}_1 \hat{n} \cdot \vec{S}_2 \hat{n} \cdot \vec{v}_1 + \frac{3}{16} \vec{S}_1 \cdot \vec{S}_2 \hat{n} \cdot \vec{v}_1 - \right. \right. \\
& \frac{15}{16} \vec{S}_1 \cdot \vec{S}_2 \hat{n} \cdot \vec{v}_1 + \frac{15}{16} \hat{n} \cdot \vec{S}_2 \hat{n} \cdot \vec{S}_1 \hat{n} \cdot \vec{v}_2 - \frac{75}{16} \hat{n} \cdot \vec{S}_1 \hat{n} \cdot \vec{S}_2 \hat{n} \cdot \vec{v}_2 + \frac{15}{16} \hat{n} \cdot \vec{v}_2 \vec{S}_1 \cdot \vec{S}_2 + \frac{3}{16} \hat{n} \cdot \vec{S}_2 \vec{S}_1 \cdot \vec{v}_1 + \\
& \frac{15}{16} \hat{n} \cdot \vec{S}_2 \vec{S}_1 \cdot \vec{v}_2 - \frac{15}{16} \hat{n} \cdot \vec{S}_1 \vec{S}_2 \cdot \vec{v}_1 - \frac{3}{16} \hat{n} \cdot \vec{S}_1 \vec{S}_2 \cdot \vec{v}_2 - \frac{3}{16} \hat{n} \cdot \vec{v}_2 \vec{S}_1 \cdot \vec{S}_2 - \frac{15}{16} \hat{n} \cdot \vec{S}_2 \vec{S}_1 \cdot \vec{v}_1 - \frac{3}{16} \hat{n} \cdot \vec{S}_2 \vec{S}_1 \cdot \vec{v}_2 + \\
& \frac{3}{16} \hat{n} \cdot \vec{S}_1 \vec{S}_2 \cdot \vec{v}_1 + \frac{15}{16} \hat{n} \cdot \vec{S}_1 \vec{S}_2 \cdot \vec{v}_2 \Big) + \frac{1}{r^5} \left( \frac{735}{32} \hat{n} \cdot \vec{S}_1 \hat{n} \cdot \vec{S}_2 \hat{n} \cdot \vec{v}_1 \hat{n} \cdot \vec{v}_2 - \frac{105}{32} \hat{n} \cdot \vec{v}_1 \vec{S}_1 \cdot \vec{S}_2 \hat{n} \cdot \vec{v}_2 - \right. \\
& \frac{105}{32} \hat{n} \cdot \vec{S}_2 \vec{S}_1 \cdot \vec{v}_1 \hat{n} \cdot \vec{v}_2 - \frac{105}{32} \hat{n} \cdot \vec{S}_1 \vec{S}_2 \cdot \vec{v}_1 \hat{n} \cdot \vec{v}_2 - \frac{105}{32} \hat{n} \cdot \vec{S}_2 \hat{n} \cdot \vec{v}_1 \vec{S}_1 \cdot \vec{v}_2 + \frac{21}{32} \vec{S}_1 \cdot \vec{v}_2 \vec{S}_2 \cdot \vec{v}_1 - \\
& \left. \frac{105}{32} \hat{n} \cdot \vec{S}_1 \hat{n} \cdot \vec{v}_1 \vec{S}_2 \cdot \vec{v}_2 + \frac{21}{32} \vec{S}_1 \cdot \vec{v}_1 \vec{S}_2 \cdot \vec{v}_2 - \frac{105}{32} \hat{n} \cdot \vec{S}_1 \hat{n} \cdot \vec{S}_2 \vec{v}_1 \cdot \vec{v}_2 + \frac{21}{32} \vec{S}_1 \cdot \vec{S}_2 \vec{v}_1 \cdot \vec{v}_2 \right) \Big) + \frac{1}{r^5} \\
& \left( -\frac{349}{2} \hat{n} \cdot \vec{S}_1 \hat{n} \cdot \vec{S}_2 (\hat{n} \cdot \vec{v}_1)^2 + \frac{35}{2} \vec{S}_1 \cdot \vec{S}_2 (\hat{n} \cdot \vec{v}_1)^2 + 456 \hat{n} \cdot \vec{S}_1 \hat{n} \cdot \vec{S}_2 \hat{n} \cdot \vec{v}_2 \hat{n} \cdot \vec{v}_1 - 30 \hat{n} \cdot \vec{v}_2 \vec{S}_1 \cdot \vec{S}_2 \hat{n} \cdot \vec{v}_1 + \right. \\
& 43 \hat{n} \cdot \vec{S}_2 \vec{S}_1 \cdot \vec{v}_1 \hat{n} \cdot \vec{v}_1 - 73 \hat{n} \cdot \vec{S}_2 \vec{S}_1 \cdot \vec{v}_2 \hat{n} \cdot \vec{v}_1 + 47 \hat{n} \cdot \vec{S}_1 \vec{S}_2 \cdot \vec{v}_1 \hat{n} \cdot \vec{v}_1 - 57 \hat{n} \cdot \vec{S}_1 \vec{S}_2 \cdot \vec{v}_2 \hat{n} \cdot \vec{v}_1 - \\
& \frac{349}{2} \hat{n} \cdot \vec{S}_1 \hat{n} \cdot \vec{S}_2 (\hat{n} \cdot \vec{v}_2)^2 + 4 \hat{n} \times \vec{S}_1 \cdot \vec{v}_1 \hat{n} \times \vec{S}_2 \cdot \vec{v}_1 - 23 \hat{n} \times \vec{S}_1 \cdot \vec{v}_2 \hat{n} \times \vec{S}_2 \cdot \vec{v}_1 - \\
& 3 \hat{n} \times \vec{S}_1 \cdot \vec{v}_1 \hat{n} \times \vec{S}_2 \cdot \vec{v}_2 + 4 \hat{n} \times \vec{S}_1 \cdot \vec{v}_2 \hat{n} \times \vec{S}_2 \cdot \vec{v}_2 + \frac{35}{2} (\hat{n} \cdot \vec{v}_2)^2 \vec{S}_1 \cdot \vec{S}_2 - 57 \hat{n} \cdot \vec{S}_2 \hat{n} \cdot \vec{v}_2 \vec{S}_1 \cdot \vec{v}_1 + \\
& 47 \hat{n} \cdot \vec{S}_2 \hat{n} \cdot \vec{v}_2 \vec{S}_1 \cdot \vec{v}_2 - 73 \hat{n} \cdot \vec{S}_1 \hat{n} \cdot \vec{v}_2 \vec{S}_2 \cdot \vec{v}_1 - 3 \vec{S}_1 \cdot \vec{v}_1 \vec{S}_2 \cdot \vec{v}_1 + 13 \vec{S}_1 \cdot \vec{v}_2 \vec{S}_2 \cdot \vec{v}_1 + \\
& 43 \hat{n} \cdot \vec{S}_1 \hat{n} \cdot \vec{v}_2 \vec{S}_2 \cdot \vec{v}_2 + \vec{S}_1 \cdot \vec{v}_1 \vec{S}_2 \cdot \vec{v}_2 - 3 \vec{S}_1 \cdot \vec{v}_2 \vec{S}_2 \cdot \vec{v}_2 + \frac{39}{2} \hat{n} \cdot \vec{S}_1 \hat{n} \cdot \vec{S}_2 \vec{v}_1 \cdot \vec{v}_1 - \frac{19}{2} \vec{S}_1 \cdot \vec{S}_2 \vec{v}_1 \cdot \vec{v}_1 - \\
& \left. 58 \hat{n} \cdot \vec{S}_1 \hat{n} \cdot \vec{S}_2 \vec{v}_1 \cdot \vec{v}_2 + 22 \vec{S}_1 \cdot \vec{S}_2 \vec{v}_1 \cdot \vec{v}_2 + \frac{39}{2} \hat{n} \cdot \vec{S}_1 \hat{n} \cdot \vec{S}_2 \vec{v}_2 \cdot \vec{v}_2 - \frac{19}{2} \vec{S}_1 \cdot \vec{S}_2 \vec{v}_2 \cdot \vec{v}_2 \right) \Big) \Big\} m_1 m_2 \Big\}
\end{aligned}$$

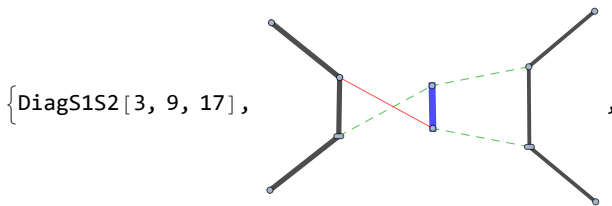

$$\begin{aligned}
& G^3 \left( \frac{-6 \hat{n} \cdot \vec{S}_2 \hat{n} \cdot \vec{S}_1 \hat{n} \cdot \vec{v}_2 - 18 \vec{S}_1 \cdot \vec{S}_2 \hat{n} \cdot \vec{v}_2 + 26 \hat{n} \cdot \vec{S}_1 \vec{S}_2 \cdot \vec{v}_2 + 10 \hat{n} \cdot \vec{S}_2 \vec{S}_1 \cdot \vec{v}_2}{r^4} + \frac{1}{r^5} \right. \\
& \pi^2 \left( -\frac{105}{32} \hat{n} \cdot \vec{S}_1 \hat{n} \cdot \vec{S}_2 (\hat{n} \cdot \vec{v}_2)^2 + \frac{15}{32} \vec{S}_1 \cdot \vec{S}_2 (\hat{n} \cdot \vec{v}_2)^2 + \frac{105}{32} \hat{n} \cdot \vec{S}_1 \hat{n} \cdot \vec{S}_2 \hat{n} \cdot \vec{v}_1 \hat{n} \cdot \vec{v}_2 - \frac{15}{32} \hat{n} \cdot \vec{v}_1 \vec{S}_1 \cdot \vec{S}_2 \hat{n} \cdot \vec{v}_2 - \right. \\
& \frac{15}{32} \hat{n} \cdot \vec{S}_2 \vec{S}_1 \cdot \vec{v}_1 \hat{n} \cdot \vec{v}_2 + \frac{15}{16} \hat{n} \cdot \vec{S}_2 \vec{S}_1 \cdot \vec{v}_2 \hat{n} \cdot \vec{v}_2 - \frac{15}{32} \hat{n} \cdot \vec{S}_1 \vec{S}_2 \cdot \vec{v}_1 \hat{n} \cdot \vec{v}_2 + \frac{15}{16} \hat{n} \cdot \vec{S}_1 \vec{S}_2 \cdot \vec{v}_2 \hat{n} \cdot \vec{v}_2 -
\end{aligned}$$

$$\begin{aligned}
& \frac{15}{32} \hat{n} \cdot \vec{S}_2 \hat{n} \cdot \vec{v}_1 \vec{S}_1 \cdot \vec{v}_2 + \frac{3}{32} \vec{S}_1 \cdot \vec{v}_2 \vec{S}_2 \cdot \vec{v}_1 - \frac{15}{32} \hat{n} \cdot \vec{S}_1 \hat{n} \cdot \vec{v}_1 \vec{S}_2 \cdot \vec{v}_2 + \frac{3}{32} \vec{S}_1 \cdot \vec{v}_1 \vec{S}_2 \cdot \vec{v}_2 - \frac{3}{16} \vec{S}_1 \cdot \vec{v}_2 \vec{S}_2 \cdot \vec{v}_2 - \\
& \frac{15}{32} \hat{n} \cdot \vec{S}_1 \hat{n} \cdot \vec{S}_2 \vec{v}_1 \cdot \vec{v}_2 + \frac{3}{32} \vec{S}_1 \cdot \vec{S}_2 \vec{v}_1 \cdot \vec{v}_2 + \frac{15}{32} \hat{n} \cdot \vec{S}_1 \hat{n} \cdot \vec{S}_2 \vec{v}_2 \cdot \vec{v}_2 - \frac{3}{32} \vec{S}_1 \cdot \vec{S}_2 \vec{v}_2 \cdot \vec{v}_2 \Big) + \frac{1}{r^5} \\
& \left( \frac{5}{2} \hat{n} \cdot \vec{S}_1 \hat{n} \cdot \vec{S}_2 (\hat{n} \cdot \vec{v}_2)^2 - \frac{87}{2} \vec{S}_1 \cdot \vec{S}_2 (\hat{n} \cdot \vec{v}_2)^2 + \frac{57}{2} \hat{n} \cdot \vec{S}_1 \hat{n} \cdot \vec{S}_2 \hat{n} \cdot \vec{v}_1 \hat{n} \cdot \vec{v}_2 + \frac{85}{2} \hat{n} \cdot \vec{v}_1 \vec{S}_1 \cdot \vec{S}_2 \hat{n} \cdot \vec{v}_2 - \right. \\
& \frac{43}{2} \hat{n} \cdot \vec{S}_2 \vec{S}_1 \cdot \vec{v}_1 \hat{n} \cdot \vec{v}_2 + 19 \hat{n} \cdot \vec{S}_2 \vec{S}_1 \cdot \vec{v}_2 \hat{n} \cdot \vec{v}_2 + \frac{9}{2} \hat{n} \cdot \vec{S}_1 \vec{S}_2 \cdot \vec{v}_1 \hat{n} \cdot \vec{v}_2 + 61 \hat{n} \cdot \vec{S}_1 \vec{S}_2 \cdot \vec{v}_2 \hat{n} \cdot \vec{v}_2 + \\
& 46 \hat{n} \times \vec{S}_1 \cdot \vec{v}_2 \hat{n} \times \vec{S}_2 \cdot \vec{v}_1 + 16 \hat{n} \times \vec{S}_1 \cdot \vec{v}_1 \hat{n} \times \vec{S}_2 \cdot \vec{v}_2 - 66 \hat{n} \times \vec{S}_1 \cdot \vec{v}_2 \hat{n} \times \vec{S}_2 \cdot \vec{v}_2 - \frac{3}{2} \hat{n} \cdot \vec{S}_2 \hat{n} \cdot \vec{v}_1 \vec{S}_1 \cdot \vec{v}_2 - \\
& \frac{9}{2} \vec{S}_1 \cdot \vec{v}_2 \vec{S}_2 \cdot \vec{v}_1 - \frac{147}{2} \hat{n} \cdot \vec{S}_1 \hat{n} \cdot \vec{v}_1 \vec{S}_2 \cdot \vec{v}_2 + \frac{55}{2} \vec{S}_1 \cdot \vec{v}_1 \vec{S}_2 \cdot \vec{v}_2 - 33 \vec{S}_1 \cdot \vec{v}_2 \vec{S}_2 \cdot \vec{v}_2 + \\
& \left. \frac{17}{2} \hat{n} \cdot \vec{S}_1 \hat{n} \cdot \vec{S}_2 \vec{v}_1 \cdot \vec{v}_2 - \frac{45}{2} \vec{S}_1 \cdot \vec{S}_2 \vec{v}_1 \cdot \vec{v}_2 + \frac{45}{2} \hat{n} \cdot \vec{S}_1 \hat{n} \cdot \vec{S}_2 \vec{v}_2 \cdot \vec{v}_2 + \frac{15}{2} \vec{S}_1 \cdot \vec{S}_2 \vec{v}_2 \cdot \vec{v}_2 \right) \Bigg\} m_1 m_2 \Bigg\}
\end{aligned}$$

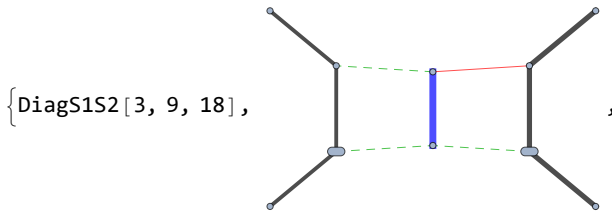

$$\begin{aligned}
& G^3 \left( \frac{384 \hat{n} \cdot \vec{a}_2 \hat{n} \cdot \vec{S}_1 \hat{n} \cdot \vec{S}_2 - 76 \vec{S}_1 \cdot \vec{a}_2 \hat{n} \cdot \vec{S}_2 - 64 \hat{n} \cdot \vec{a}_2 \vec{S}_1 \cdot \vec{S}_2 - 60 \hat{n} \cdot \vec{S}_1 \vec{S}_2 \cdot \vec{a}_2}{r^4} + \right. \\
& \frac{1}{r^5} \left( \frac{387}{2} \hat{n} \cdot \vec{S}_1 \hat{n} \cdot \vec{S}_2 (\hat{n} \cdot \vec{v}_2)^2 - \frac{153}{2} \vec{S}_1 \cdot \vec{S}_2 (\hat{n} \cdot \vec{v}_2)^2 - \frac{387}{2} \hat{n} \cdot \vec{S}_1 \hat{n} \cdot \vec{S}_2 \hat{n} \cdot \vec{v}_1 \hat{n} \cdot \vec{v}_2 + \right. \\
& \frac{153}{2} \hat{n} \cdot \vec{v}_1 \vec{S}_1 \cdot \vec{S}_2 \hat{n} \cdot \vec{v}_2 - \frac{31}{2} \hat{n} \cdot \vec{S}_2 \vec{S}_1 \cdot \vec{v}_1 \hat{n} \cdot \vec{v}_2 - 3 \hat{n} \cdot \vec{S}_2 \vec{S}_1 \cdot \vec{v}_2 \hat{n} \cdot \vec{v}_2 - \frac{51}{2} \hat{n} \cdot \vec{S}_1 \vec{S}_2 \cdot \vec{v}_1 \hat{n} \cdot \vec{v}_2 + \\
& 7 \hat{n} \cdot \vec{S}_1 \vec{S}_2 \cdot \vec{v}_2 \hat{n} \cdot \vec{v}_2 + 14 \hat{n} \times \vec{S}_1 \cdot \vec{v}_2 \hat{n} \times \vec{S}_2 \cdot \vec{v}_1 + 44 \hat{n} \times \vec{S}_1 \cdot \vec{v}_1 \hat{n} \times \vec{S}_2 \cdot \vec{v}_2 - 58 \hat{n} \times \vec{S}_1 \cdot \vec{v}_2 \hat{n} \times \vec{S}_2 \cdot \vec{v}_2 + \\
& \frac{17}{2} \hat{n} \cdot \vec{S}_2 \hat{n} \cdot \vec{v}_1 \vec{S}_1 \cdot \vec{v}_2 + \frac{59}{2} \vec{S}_1 \cdot \vec{v}_2 \vec{S}_2 \cdot \vec{v}_1 + \frac{57}{2} \hat{n} \cdot \vec{S}_1 \hat{n} \cdot \vec{v}_1 \vec{S}_2 \cdot \vec{v}_2 + \frac{19}{2} \vec{S}_1 \cdot \vec{v}_1 \vec{S}_2 \cdot \vec{v}_2 - 39 \vec{S}_1 \cdot \vec{v}_2 \vec{S}_2 \cdot \vec{v}_2 + \\
& \left. \frac{37}{2} \hat{n} \cdot \vec{S}_1 \hat{n} \cdot \vec{S}_2 \vec{v}_1 \cdot \vec{v}_2 - \frac{89}{2} \vec{S}_1 \cdot \vec{S}_2 \vec{v}_1 \cdot \vec{v}_2 - \frac{37}{2} \hat{n} \cdot \vec{S}_1 \hat{n} \cdot \vec{S}_2 \vec{v}_2 \cdot \vec{v}_2 + \frac{89}{2} \vec{S}_1 \cdot \vec{S}_2 \vec{v}_2 \cdot \vec{v}_2 \right) + \\
& \left. \pi^2 \left( \frac{-\frac{45}{2} \hat{n} \cdot \vec{a}_2 \hat{n} \cdot \vec{S}_1 \hat{n} \cdot \vec{S}_2 + \frac{9}{2} \vec{S}_1 \cdot \vec{a}_2 \hat{n} \cdot \vec{S}_2 + \frac{9}{2} \hat{n} \cdot \vec{a}_2 \vec{S}_1 \cdot \vec{S}_2 + \frac{9}{2} \hat{n} \cdot \vec{S}_1 \vec{S}_2 \cdot \vec{a}_2}{r^4} + \frac{1}{r^5} \right. \right. \\
& \left( -\frac{315}{32} \hat{n} \cdot \vec{S}_1 \hat{n} \cdot \vec{S}_2 (\hat{n} \cdot \vec{v}_2)^2 + \frac{45}{32} \vec{S}_1 \cdot \vec{S}_2 (\hat{n} \cdot \vec{v}_2)^2 + \frac{315}{32} \hat{n} \cdot \vec{S}_1 \hat{n} \cdot \vec{S}_2 \hat{n} \cdot \vec{v}_1 \hat{n} \cdot \vec{v}_2 - \frac{45}{32} \hat{n} \cdot \vec{v}_1 \vec{S}_1 \cdot \vec{S}_2 \hat{n} \cdot \vec{v}_2 - \right. \\
& \frac{45}{32} \hat{n} \cdot \vec{S}_2 \vec{S}_1 \cdot \vec{v}_1 \hat{n} \cdot \vec{v}_2 + \frac{45}{16} \hat{n} \cdot \vec{S}_2 \vec{S}_1 \cdot \vec{v}_2 \hat{n} \cdot \vec{v}_2 - \frac{45}{32} \hat{n} \cdot \vec{S}_1 \vec{S}_2 \cdot \vec{v}_1 \hat{n} \cdot \vec{v}_2 + \frac{45}{16} \hat{n} \cdot \vec{S}_1 \vec{S}_2 \cdot \vec{v}_2 \hat{n} \cdot \vec{v}_2 - \\
& \frac{45}{32} \hat{n} \cdot \vec{S}_2 \hat{n} \cdot \vec{v}_1 \vec{S}_1 \cdot \vec{v}_2 + \frac{9}{32} \vec{S}_1 \cdot \vec{v}_2 \vec{S}_2 \cdot \vec{v}_1 - \frac{45}{32} \hat{n} \cdot \vec{S}_1 \hat{n} \cdot \vec{v}_1 \vec{S}_2 \cdot \vec{v}_2 + \frac{9}{32} \vec{S}_1 \cdot \vec{v}_1 \vec{S}_2 \cdot \vec{v}_2 - \frac{9}{16} \vec{S}_1 \cdot \vec{v}_2 \vec{S}_2 \cdot \vec{v}_2 - \\
& \left. \left. \frac{45}{32} \hat{n} \cdot \vec{S}_1 \hat{n} \cdot \vec{S}_2 \vec{v}_1 \cdot \vec{v}_2 + \frac{9}{32} \vec{S}_1 \cdot \vec{S}_2 \vec{v}_1 \cdot \vec{v}_2 + \frac{45}{32} \hat{n} \cdot \vec{S}_1 \hat{n} \cdot \vec{S}_2 \vec{v}_2 \cdot \vec{v}_2 - \frac{9}{32} \vec{S}_1 \cdot \vec{S}_2 \vec{v}_2 \cdot \vec{v}_2 \right) \right) \Bigg\} m_1 m_2 \Bigg\}
\end{aligned}$$

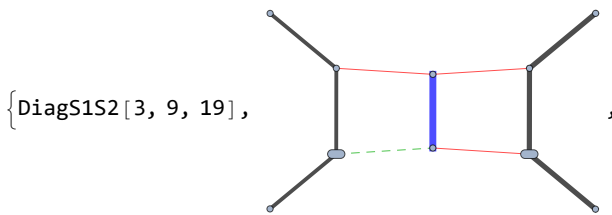

$$G^3 m_1 m_2 \left\{ \frac{-20 \vec{S}_1 \cdot \vec{S}_2 \hat{n} \cdot \vec{a}_1 + 20 \vec{S}_2 \cdot \vec{a}_1 \hat{n} \cdot \vec{S}_1 - 20 \vec{S}_1 \cdot \vec{S}_2 \hat{n} \cdot \vec{v}_1 + 20 \hat{n} \cdot \vec{S}_1 \vec{S}_2 \cdot \vec{v}_1 - 20 \vec{S}_1 \cdot \vec{S}_2 \hat{n} \cdot \vec{v}_1 + 20 \hat{n} \cdot \vec{S}_1 \vec{S}_2 \cdot \vec{v}_1}{r^4} + \right.$$

$$\left. \frac{1}{r^5} \left( -54 \hat{n} \times \vec{S}_1 \cdot \vec{v}_1 \hat{n} \times \vec{S}_2 \cdot \vec{v}_1 + 50 \hat{n} \times \vec{S}_1 \cdot \vec{v}_1 \hat{n} \times \vec{S}_2 \cdot \vec{v}_2 + 54 \vec{S}_1 \cdot \vec{S}_2 (\hat{n} \cdot \vec{v}_1)^2 - 60 \vec{S}_1 \cdot \vec{S}_2 \hat{n} \cdot \vec{v}_2 \hat{n} \cdot \vec{v}_1 - \right. \right.$$

$$\left. \left. 54 \hat{n} \cdot \vec{S}_1 \hat{n} \cdot \vec{v}_1 \vec{S}_2 \cdot \vec{v}_1 + 60 \hat{n} \cdot \vec{S}_1 \hat{n} \cdot \vec{v}_2 \vec{S}_2 \cdot \vec{v}_1 - 6 \vec{S}_1 \cdot \vec{v}_2 \vec{S}_2 \cdot \vec{v}_1 + 6 \vec{S}_1 \cdot \vec{S}_2 \vec{v}_1 \cdot \vec{v}_2 \right) \right\}$$

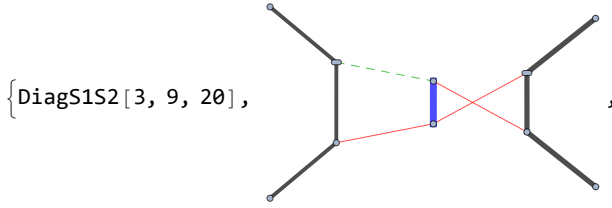

$$G^3 m_1 m_2 \left\{ \frac{1}{r^5} \left( -46 \hat{n} \times \vec{S}_1 \cdot \vec{v}_1 \hat{n} \times \vec{S}_2 \cdot \vec{v}_1 + 70 \hat{n} \times \vec{S}_1 \cdot \vec{v}_1 \hat{n} \times \vec{S}_2 \cdot \vec{v}_2 - 54 \vec{S}_1 \cdot \vec{S}_2 (\hat{n} \cdot \vec{v}_1)^2 + \right. \right.$$

$$60 \vec{S}_1 \cdot \vec{S}_2 \hat{n} \cdot \vec{v}_2 \hat{n} \cdot \vec{v}_1 + 54 \hat{n} \cdot \vec{S}_1 \hat{n} \cdot \vec{v}_1 \vec{S}_2 \cdot \vec{v}_1 - 60 \hat{n} \cdot \vec{S}_1 \hat{n} \cdot \vec{v}_2 \vec{S}_2 \cdot \vec{v}_1 - 20 \vec{S}_1 \cdot \vec{v}_1 \vec{S}_2 \cdot \vec{v}_1 +$$

$$30 \vec{S}_1 \cdot \vec{v}_2 \vec{S}_2 \cdot \vec{v}_1 + 20 \vec{S}_1 \cdot \vec{S}_2 \vec{v}_1 \cdot \vec{v}_1 - 30 \vec{S}_1 \cdot \vec{S}_2 \vec{v}_1 \cdot \vec{v}_2 \left. \right) + \frac{20 \vec{S}_1 \cdot \vec{S}_2 \hat{n} \cdot \vec{v}_1 - 20 \hat{n} \cdot \vec{S}_1 \vec{S}_2 \cdot \vec{v}_1}{r^4} \left. \right\}$$

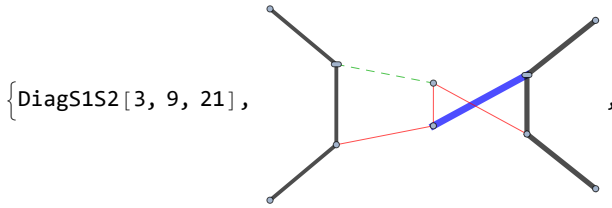

$$G^3 m_1 m_2 \left\{ \frac{\frac{5}{2} \hat{n} \cdot \vec{a}_1 \hat{n} \cdot \vec{S}_1 \hat{n} \cdot \vec{S}_2 - \frac{3}{2} \vec{S}_1 \cdot \vec{S}_2 \hat{n} \cdot \vec{a}_1 - \vec{S}_2 \cdot \vec{a}_1 \hat{n} \cdot \vec{S}_1 + \frac{5}{2} \hat{n} \cdot \vec{S}_1 \hat{n} \cdot \vec{S}_2 \hat{n} \cdot \vec{v}_1 - \frac{3}{2} \vec{S}_1 \cdot \vec{S}_2 \hat{n} \cdot \vec{v}_1 - \hat{n} \cdot \vec{S}_1 \vec{S}_2 \cdot \vec{v}_1}{r^4} + \right.$$

$$\frac{1}{r^5} \left( 4 \hat{n} \times \vec{S}_1 \cdot \vec{v}_1 \hat{n} \times \vec{S}_2 \cdot \vec{v}_1 - \frac{1}{4} \hat{n} \times \vec{S}_1 \cdot \vec{v}_2 \hat{n} \times \vec{S}_2 \cdot \vec{v}_1 - \frac{1}{4} \hat{n} \times \vec{S}_1 \cdot \vec{v}_1 \hat{n} \times \vec{S}_2 \cdot \vec{v}_2 + \frac{1}{2} \hat{n} \cdot \vec{S}_1 \hat{n} \cdot \vec{S}_2 (\hat{n} \cdot \vec{v}_1)^2 - \right.$$

$$\frac{1}{2} \vec{S}_1 \cdot \vec{S}_2 (\hat{n} \cdot \vec{v}_1)^2 + \frac{49}{4} \hat{n} \cdot \vec{S}_1 \hat{n} \cdot \vec{S}_2 \hat{n} \cdot \vec{v}_2 \hat{n} \cdot \vec{v}_1 - \frac{29}{4} \vec{S}_1 \cdot \vec{S}_2 \hat{n} \cdot \vec{v}_2 \hat{n} \cdot \vec{v}_1 - \frac{5}{2} \hat{n} \cdot \vec{S}_2 \hat{n} \cdot \vec{v}_1 \vec{S}_1 \cdot \vec{v}_1 +$$

$$\frac{5}{2} \hat{n} \cdot \vec{S}_1 \hat{n} \cdot \vec{v}_1 \vec{S}_2 \cdot \vec{v}_1 - \frac{5}{2} \hat{n} \cdot \vec{S}_1 \hat{n} \cdot \vec{v}_1 \vec{S}_2 \cdot \vec{v}_2 - \frac{5}{2} \hat{n} \cdot \vec{S}_1 \hat{n} \cdot \vec{v}_2 \vec{S}_2 \cdot \vec{v}_1 + \frac{1}{2} \vec{v}_1 \cdot \vec{v}_1 \hat{n} \cdot \vec{S}_1 \hat{n} \cdot \vec{S}_2 -$$

$$\left. \left. \frac{9}{4} \vec{v}_1 \cdot \vec{v}_2 \hat{n} \cdot \vec{S}_1 \hat{n} \cdot \vec{S}_2 + \vec{S}_1 \cdot \vec{v}_1 \vec{S}_2 \cdot \vec{v}_1 - \frac{3}{2} \vec{S}_1 \cdot \vec{S}_2 \vec{v}_1 \cdot \vec{v}_1 + \frac{9}{4} \vec{S}_1 \cdot \vec{S}_2 \vec{v}_1 \cdot \vec{v}_2 \right) \right\}$$

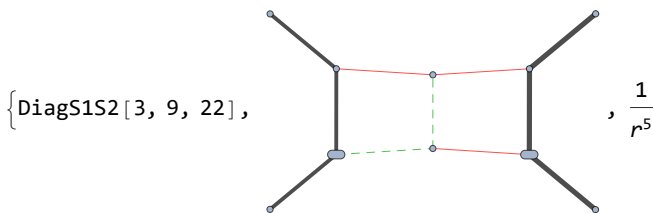

$$G^3 m_1 m_2 \left( 10 \hat{n} \times \vec{S}_1 \cdot \vec{v}_1 \hat{n} \times \vec{S}_2 \cdot \vec{v}_1 - 14 \hat{n} \times \vec{S}_1 \cdot \vec{v}_1 \hat{n} \times \vec{S}_2 \cdot \vec{v}_2 + 10 \vec{S}_1 \cdot \vec{S}_2 (\hat{n} \cdot \vec{v}_1)^2 - \right.$$



$$10 \hat{n} \cdot \vec{S}_1 \hat{n} \cdot \vec{v}_1 \vec{S}_2 \cdot \vec{v}_1 + 4 \vec{S}_1 \cdot \vec{v}_1 \vec{S}_2 \cdot \vec{v}_1 - 6 \vec{S}_1 \cdot \vec{v}_2 \vec{S}_2 \cdot \vec{v}_1 - 4 \vec{S}_1 \cdot \vec{S}_2 \vec{v}_1 \cdot \vec{v}_1 + 6 \vec{S}_1 \cdot \vec{S}_2 \vec{v}_1 \cdot \vec{v}_2 \Big) \Big\}$$

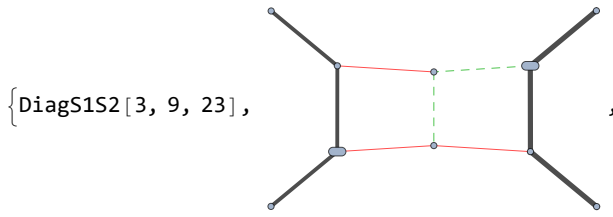

$$G^3 m_1 m_2 \left( \frac{4 \vec{S}_1 \cdot \vec{a}_2 \hat{n} \cdot \vec{S}_2 - 4 \vec{S}_1 \cdot \vec{S}_2 \hat{n} \cdot \vec{a}_2 - 4 \vec{S}_1 \cdot \vec{S}_2 \hat{n} \cdot \vec{v}_2 + 4 \hat{n} \cdot \vec{S}_2 \vec{S}_1 \cdot \vec{v}_2}{r^4} + \frac{1}{r^5} \left( -6 \hat{n} \times \vec{S}_1 \cdot \vec{v}_1 \hat{n} \times \vec{S}_2 \cdot \vec{v}_2 + \right. \right. \\ \left. \left. 10 \hat{n} \times \vec{S}_1 \cdot \vec{v}_2 \hat{n} \times \vec{S}_2 \cdot \vec{v}_2 - 10 \vec{S}_1 \cdot \vec{S}_2 (\hat{n} \cdot \vec{v}_2)^2 + 10 \hat{n} \cdot \vec{S}_2 \hat{n} \cdot \vec{v}_2 \vec{S}_1 \cdot \vec{v}_2 + 2 \vec{S}_1 \cdot \vec{v}_2 \vec{S}_2 \cdot \vec{v}_1 - 2 \vec{S}_1 \cdot \vec{S}_2 \vec{v}_1 \cdot \vec{v}_2 \right) \right) \Big\}$$

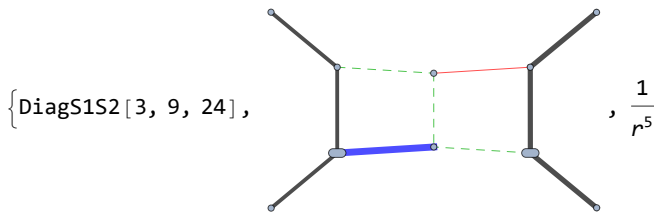

$$G^3 m_1 m_2 \left( -4 \hat{n} \times \vec{S}_1 \cdot \vec{v}_2 \hat{n} \times \vec{S}_2 \cdot \vec{v}_2 + 49 \hat{n} \cdot \vec{S}_1 \hat{n} \cdot \vec{S}_2 (\hat{n} \cdot \vec{v}_2)^2 - 5 \vec{S}_1 \cdot \vec{S}_2 (\hat{n} \cdot \vec{v}_2)^2 - \right. \\ \left. 18 \hat{n} \cdot \vec{S}_2 \hat{n} \cdot \vec{v}_2 \vec{S}_1 \cdot \vec{v}_2 - 24 \hat{n} \cdot \vec{S}_1 \hat{n} \cdot \vec{v}_2 \vec{S}_2 \cdot \vec{v}_2 - 15 \vec{v}_2 \cdot \vec{v}_2 \hat{n} \cdot \vec{S}_1 \hat{n} \cdot \vec{S}_2 + 8 \vec{S}_1 \cdot \vec{v}_2 \vec{S}_2 \cdot \vec{v}_2 + 5 \vec{S}_1 \cdot \vec{S}_2 \vec{v}_2 \cdot \vec{v}_2 \right) \Big\}$$

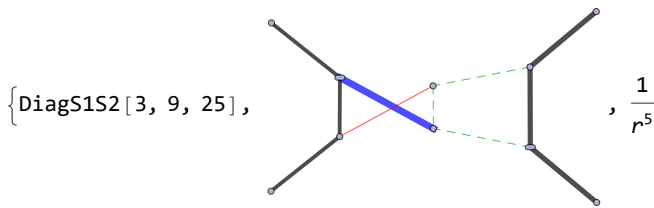

$$G^3 m_1 m_2 \left( -4 \hat{n} \times \vec{S}_1 \cdot \vec{v}_2 \hat{n} \times \vec{S}_2 \cdot \vec{v}_1 + 8 \hat{n} \times \vec{S}_1 \cdot \vec{v}_1 \hat{n} \times \vec{S}_2 \cdot \vec{v}_2 - 49 \hat{n} \cdot \vec{S}_1 \hat{n} \cdot \vec{S}_2 \hat{n} \cdot \vec{v}_1 \hat{n} \cdot \vec{v}_2 + \right. \\ \left. 5 \vec{S}_1 \cdot \vec{S}_2 \hat{n} \cdot \vec{v}_1 \hat{n} \cdot \vec{v}_2 + 11 \hat{n} \cdot \vec{S}_2 \hat{n} \cdot \vec{v}_2 \vec{S}_1 \cdot \vec{v}_1 + 7 \hat{n} \cdot \vec{S}_2 \hat{n} \cdot \vec{v}_1 \vec{S}_1 \cdot \vec{v}_2 + 23 \hat{n} \cdot \vec{S}_1 \hat{n} \cdot \vec{v}_2 \vec{S}_2 \cdot \vec{v}_1 + \right. \\ \left. \hat{n} \cdot \vec{S}_1 \hat{n} \cdot \vec{v}_1 \vec{S}_2 \cdot \vec{v}_2 + 15 \vec{v}_1 \cdot \vec{v}_2 \hat{n} \cdot \vec{S}_1 \hat{n} \cdot \vec{S}_2 - 7 \vec{S}_1 \cdot \vec{v}_2 \vec{S}_2 \cdot \vec{v}_1 - \vec{S}_1 \cdot \vec{v}_1 \vec{S}_2 \cdot \vec{v}_2 - 5 \vec{S}_1 \cdot \vec{S}_2 \vec{v}_1 \cdot \vec{v}_2 \right) \Big\}$$

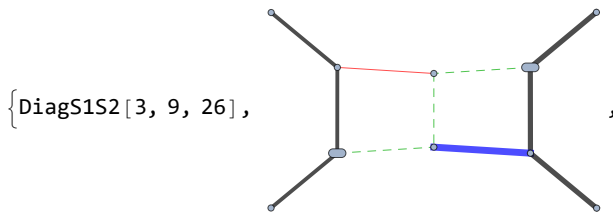

$$G^3 m_1 m_2 \left( \frac{1}{r^5} \left( 10 \hat{n} \times \vec{S}_1 \cdot \vec{v}_1 \hat{n} \times \vec{S}_2 \cdot \vec{v}_1 + 108 \hat{n} \cdot \vec{S}_1 \hat{n} \cdot \vec{S}_2 (\hat{n} \cdot \vec{v}_1)^2 - 14 \vec{S}_1 \cdot \vec{S}_2 (\hat{n} \cdot \vec{v}_1)^2 - \right. \right. \\ \left. \left. 50 \hat{n} \cdot \vec{S}_2 \hat{n} \cdot \vec{v}_1 \vec{S}_1 \cdot \vec{v}_1 - 24 \hat{n} \cdot \vec{S}_1 \hat{n} \cdot \vec{v}_1 \vec{S}_2 \cdot \vec{v}_1 - 4 \vec{v}_1 \cdot \vec{v}_1 \hat{n} \cdot \vec{S}_1 \hat{n} \cdot \vec{S}_2 + 12 \vec{S}_1 \cdot \vec{v}_1 \vec{S}_2 \cdot \vec{v}_1 - 4 \vec{S}_1 \cdot \vec{S}_2 \vec{v}_1 \cdot \vec{v}_1 \right) + \right. \\ \left. \frac{1}{r^5} \pi^2 \left( \frac{1155}{32} \hat{n} \cdot \vec{S}_1 \hat{n} \cdot \vec{S}_2 (\hat{n} \cdot \vec{v}_1)^2 - \frac{165}{32} \vec{S}_1 \cdot \vec{S}_2 (\hat{n} \cdot \vec{v}_1)^2 - \frac{165}{16} \hat{n} \cdot \vec{S}_2 \hat{n} \cdot \vec{v}_1 \vec{S}_1 \cdot \vec{v}_1 - \right. \right. \\ \left. \left. \frac{165}{16} \hat{n} \cdot \vec{S}_1 \hat{n} \cdot \vec{v}_1 \vec{S}_2 \cdot \vec{v}_1 - \frac{165}{32} \vec{v}_1 \cdot \vec{v}_1 \hat{n} \cdot \vec{S}_1 \hat{n} \cdot \vec{S}_2 + \frac{33}{16} \vec{S}_1 \cdot \vec{v}_1 \vec{S}_2 \cdot \vec{v}_1 + \frac{33}{32} \vec{S}_1 \cdot \vec{S}_2 \vec{v}_1 \cdot \vec{v}_1 \right) \right) \Big\}$$

{DiagS1S2 [3, 9, 27],

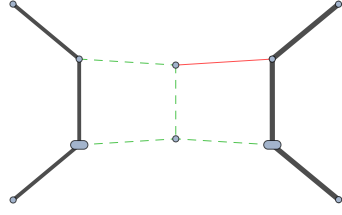

,

$$\begin{aligned}
 & G^3 \left( \frac{1}{r^4} \left( -20 \hat{n} \cdot \vec{a}_2 \hat{n} \cdot \vec{S}_1 \hat{n} \cdot \vec{S}_2 + 10 \hat{n} \cdot \vec{S}_1 \hat{n} \cdot \vec{v}_2 \hat{n} \cdot \vec{S}_2 + 8 \vec{S}_1 \cdot \vec{v}_2 \hat{n} \cdot \vec{S}_2 - 6 \vec{S}_1 \cdot \vec{a}_2 \hat{n} \cdot \vec{S}_2 + 10 \hat{n} \cdot \vec{S}_2 \hat{n} \cdot \vec{S}_1 \hat{n} \cdot \vec{v}_2 - 8 \hat{n} \cdot \vec{v}_2 \right. \right. \\
 & \quad \left. \left. \vec{S}_1 \cdot \vec{S}_2 + 8 \hat{n} \cdot \vec{S}_1 \vec{S}_2 \cdot \vec{v}_2 - 8 \hat{n} \cdot \vec{v}_2 \vec{S}_1 \cdot \vec{S}_2 + 16 \hat{n} \cdot \vec{a}_2 \vec{S}_1 \cdot \vec{S}_2 - 2 \hat{n} \cdot \vec{S}_2 \vec{S}_1 \cdot \vec{v}_2 - 6 \hat{n} \cdot \vec{S}_1 \vec{S}_2 \cdot \vec{a}_2 - 2 \hat{n} \cdot \vec{S}_1 \vec{S}_2 \cdot \vec{v}_2 \right) + \frac{1}{r^5} \right. \\
 & \quad \left( -\frac{65}{2} \hat{n} \cdot \vec{S}_1 \hat{n} \cdot \vec{S}_2 (\hat{n} \cdot \vec{v}_2)^2 + \frac{59}{2} \vec{S}_1 \cdot \vec{S}_2 (\hat{n} \cdot \vec{v}_2)^2 + \frac{65}{2} \hat{n} \cdot \vec{S}_1 \hat{n} \cdot \vec{S}_2 \hat{n} \cdot \vec{v}_1 \hat{n} \cdot \vec{v}_2 - \frac{59}{2} \hat{n} \cdot \vec{v}_1 \vec{S}_1 \cdot \vec{S}_2 \hat{n} \cdot \vec{v}_2 + \right. \\
 & \quad \left. \frac{19}{2} \hat{n} \cdot \vec{S}_2 \vec{S}_1 \cdot \vec{v}_1 \hat{n} \cdot \vec{v}_2 - 27 \hat{n} \cdot \vec{S}_2 \vec{S}_1 \cdot \vec{v}_2 \hat{n} \cdot \vec{v}_2 + \frac{11}{2} \hat{n} \cdot \vec{S}_1 \vec{S}_2 \cdot \vec{v}_1 \hat{n} \cdot \vec{v}_2 + 9 \hat{n} \cdot \vec{S}_1 \vec{S}_2 \cdot \vec{v}_2 \hat{n} \cdot \vec{v}_2 - \right. \\
 & \quad \left. 11 \hat{n} \times \vec{S}_1 \cdot \vec{v}_2 \hat{n} \times \vec{S}_2 \cdot \vec{v}_1 - 21 \hat{n} \times \vec{S}_1 \cdot \vec{v}_1 \hat{n} \times \vec{S}_2 \cdot \vec{v}_2 + 32 \hat{n} \times \vec{S}_1 \cdot \vec{v}_2 \hat{n} \times \vec{S}_2 \cdot \vec{v}_2 - \frac{37}{2} \hat{n} \cdot \vec{S}_2 \hat{n} \cdot \vec{v}_1 \vec{S}_1 \cdot \vec{v}_2 + \right. \\
 & \quad \left. \frac{1}{2} \vec{S}_1 \cdot \vec{v}_2 \vec{S}_2 \cdot \vec{v}_1 + \frac{43}{2} \hat{n} \cdot \vec{S}_1 \hat{n} \cdot \vec{v}_1 \vec{S}_2 \cdot \vec{v}_2 - \frac{19}{2} \vec{S}_1 \cdot \vec{v}_1 \vec{S}_2 \cdot \vec{v}_2 + 9 \vec{S}_1 \cdot \vec{v}_2 \vec{S}_2 \cdot \vec{v}_2 - \right. \\
 & \quad \left. \frac{35}{2} \hat{n} \cdot \vec{S}_1 \hat{n} \cdot \vec{S}_2 \vec{v}_1 \cdot \vec{v}_2 + \frac{35}{2} \vec{S}_1 \cdot \vec{S}_2 \vec{v}_1 \cdot \vec{v}_2 + \frac{35}{2} \hat{n} \cdot \vec{S}_1 \hat{n} \cdot \vec{S}_2 \vec{v}_2 \cdot \vec{v}_2 - \frac{35}{2} \vec{S}_1 \cdot \vec{S}_2 \vec{v}_2 \cdot \vec{v}_2 \right) + \\
 & \quad \pi^2 \left( \frac{1}{r^4} \left( -\frac{15}{2} \hat{n} \cdot \vec{S}_2 \hat{n} \cdot \vec{S}_1 \hat{n} \cdot \vec{v}_2 + \frac{15}{4} \hat{n} \cdot \vec{S}_1 \hat{n} \cdot \vec{S}_2 \hat{n} \cdot \vec{v}_2 - \frac{3}{4} \vec{S}_1 \cdot \vec{S}_2 \hat{n} \cdot \vec{v}_2 + \frac{3}{2} \vec{S}_1 \cdot \vec{S}_2 \hat{n} \cdot \vec{v}_2 - \right. \right. \\
 & \quad \left. \left. \frac{3}{4} \hat{n} \cdot \vec{S}_2 \vec{S}_1 \cdot \vec{v}_2 + \frac{3}{2} \hat{n} \cdot \vec{S}_1 \vec{S}_2 \cdot \vec{v}_2 + \frac{3}{2} \hat{n} \cdot \vec{S}_2 \vec{S}_1 \cdot \vec{v}_2 - \frac{3}{4} \hat{n} \cdot \vec{S}_1 \vec{S}_2 \cdot \vec{v}_2 \right) + \frac{1}{r^5} \right. \\
 & \quad \left( -\frac{945}{32} \hat{n} \cdot \vec{S}_1 \hat{n} \cdot \vec{S}_2 (\hat{n} \cdot \vec{v}_2)^2 + \frac{135}{32} \vec{S}_1 \cdot \vec{S}_2 (\hat{n} \cdot \vec{v}_2)^2 - \frac{945}{32} \hat{n} \cdot \vec{S}_1 \hat{n} \cdot \vec{S}_2 \hat{n} \cdot \vec{v}_1 \hat{n} \cdot \vec{v}_2 + \frac{135}{32} \hat{n} \cdot \vec{v}_1 \vec{S}_1 \cdot \vec{S}_2 \hat{n} \cdot \vec{v}_2 + \right. \\
 & \quad \frac{135}{32} \hat{n} \cdot \vec{S}_2 \vec{S}_1 \cdot \vec{v}_1 \hat{n} \cdot \vec{v}_2 + \frac{135}{16} \hat{n} \cdot \vec{S}_2 \vec{S}_1 \cdot \vec{v}_2 \hat{n} \cdot \vec{v}_2 + \frac{135}{32} \hat{n} \cdot \vec{S}_1 \vec{S}_2 \cdot \vec{v}_1 \hat{n} \cdot \vec{v}_2 + \frac{135}{16} \hat{n} \cdot \vec{S}_1 \vec{S}_2 \cdot \vec{v}_2 \hat{n} \cdot \vec{v}_2 + \\
 & \quad \frac{135}{32} \hat{n} \cdot \vec{S}_2 \hat{n} \cdot \vec{v}_1 \vec{S}_1 \cdot \vec{v}_2 - \frac{27}{32} \vec{S}_1 \cdot \vec{v}_2 \vec{S}_2 \cdot \vec{v}_1 + \frac{135}{32} \hat{n} \cdot \vec{S}_1 \hat{n} \cdot \vec{v}_1 \vec{S}_2 \cdot \vec{v}_2 - \frac{27}{32} \vec{S}_1 \cdot \vec{v}_1 \vec{S}_2 \cdot \vec{v}_2 - \frac{27}{16} \vec{S}_1 \cdot \vec{v}_2 \vec{S}_2 \cdot \vec{v}_2 + \\
 & \quad \left. \left. \frac{135}{32} \hat{n} \cdot \vec{S}_1 \hat{n} \cdot \vec{S}_2 \vec{v}_1 \cdot \vec{v}_2 - \frac{27}{32} \vec{S}_1 \cdot \vec{S}_2 \vec{v}_1 \cdot \vec{v}_2 + \frac{135}{32} \hat{n} \cdot \vec{S}_1 \hat{n} \cdot \vec{S}_2 \vec{v}_2 \cdot \vec{v}_2 - \frac{27}{32} \vec{S}_1 \cdot \vec{S}_2 \vec{v}_2 \cdot \vec{v}_2 \right) \right) \left. \right) m_1 m_2 \}
 \end{aligned}$$

{DiagS1S2 [3, 9, 28],

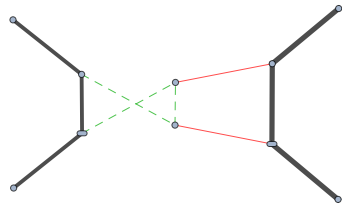

,

$$\frac{G^3 m_1 m_2 \left( -40 \hat{n} \times \vec{S}_1 \cdot \vec{v}_1 \hat{n} \times \vec{S}_2 \cdot \vec{v}_2 - 8 \vec{S}_1 \cdot \vec{S}_2 \hat{n} \cdot \vec{v}_1 \hat{n} \cdot \vec{v}_2 + 8 \hat{n} \cdot \vec{S}_1 \hat{n} \cdot \vec{v}_2 \vec{S}_2 \cdot \vec{v}_1 - 16 \vec{S}_1 \cdot \vec{v}_2 \vec{S}_2 \cdot \vec{v}_1 + 16 \vec{S}_1 \cdot \vec{S}_2 \vec{v}_1 \cdot \vec{v}_2 \right)}{r^5}$$

{DiagS1S2 [3, 9, 29],

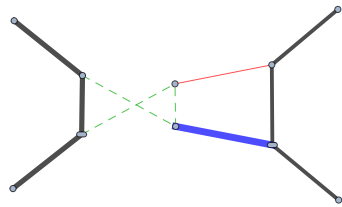

,  $\frac{1}{r^5}$

$$\begin{aligned}
 & G^3 m_1 m_2 \left( -18 \hat{n} \times \vec{S}_1 \cdot \vec{v}_2 \hat{n} \times \vec{S}_2 \cdot \vec{v}_1 + 24 \hat{n} \times \vec{S}_1 \cdot \vec{v}_1 \hat{n} \times \vec{S}_2 \cdot \vec{v}_2 + 52 \hat{n} \cdot \vec{S}_1 \hat{n} \cdot \vec{S}_2 \hat{n} \cdot \vec{v}_1 \hat{n} \cdot \vec{v}_2 - \right. \\
 & \quad \left. 18 \vec{S}_1 \cdot \vec{S}_2 \hat{n} \cdot \vec{v}_1 \hat{n} \cdot \vec{v}_2 - 10 \hat{n} \cdot \vec{S}_2 \hat{n} \cdot \vec{v}_2 \vec{S}_1 \cdot \vec{v}_1 - 12 \hat{n} \cdot \vec{S}_2 \hat{n} \cdot \vec{v}_1 \vec{S}_1 \cdot \vec{v}_2 - 12 \hat{n} \cdot \vec{S}_1 \hat{n} \cdot \vec{v}_2 \vec{S}_2 \cdot \vec{v}_1 + \right.
 \end{aligned}$$

$$8 \vec{v}_1 \cdot \vec{v}_2 \hat{n} \cdot \vec{S}_1 \hat{n} \cdot \vec{S}_2 + 12 \vec{S}_1 \cdot \vec{v}_2 \vec{S}_2 \cdot \vec{v}_1 - 4 \vec{S}_1 \cdot \vec{v}_1 \vec{S}_2 \cdot \vec{v}_2 - 8 \vec{S}_1 \cdot \vec{S}_2 \vec{v}_1 \cdot \vec{v}_2 \Big) \Big\}$$

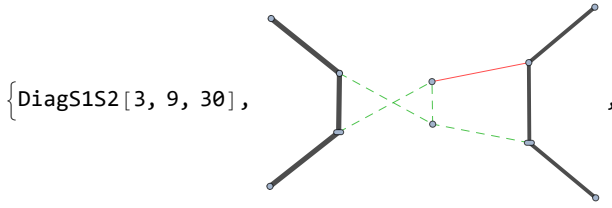

$$\begin{aligned} G^3 \Bigg( & \frac{1}{r^4} \left( 10 \hat{n} \cdot \vec{a}_1 \hat{n} \cdot \vec{S}_1 \hat{n} \cdot \vec{S}_2 + 2 \hat{n} \cdot \vec{S}_1 \hat{n} \cdot \vec{v}_1 \hat{n} \cdot \vec{S}_2 - 6 \vec{S}_1 \cdot \vec{v}_1 \hat{n} \cdot \vec{S}_2 + 4 \vec{S}_1 \cdot \vec{a}_1 \hat{n} \cdot \vec{S}_2 - 4 \hat{n} \cdot \vec{S}_2 \hat{n} \cdot \vec{S}_1 \hat{n} \cdot \vec{v}_1 + \right. \\ & 14 \hat{n} \cdot \vec{v}_1 \vec{S}_1 \cdot \vec{S}_2 + 2 \hat{n} \cdot \vec{S}_1 \vec{S}_2 \cdot \vec{v}_1 - 12 \hat{n} \cdot \vec{a}_1 \vec{S}_1 \cdot \vec{S}_2 + 2 \hat{n} \cdot \vec{S}_2 \vec{S}_1 \cdot \vec{v}_1 - 2 \hat{n} \cdot \vec{S}_1 \vec{S}_2 \cdot \vec{a}_1 - 2 \hat{n} \cdot \vec{S}_1 \vec{S}_2 \cdot \vec{v}_1 \Big) + \frac{1}{r^5} \\ & \left( -\frac{91}{2} \hat{n} \cdot \vec{S}_1 \hat{n} \cdot \vec{S}_2 (\hat{n} \cdot \vec{v}_1)^2 - \frac{71}{2} \vec{S}_1 \cdot \vec{S}_2 (\hat{n} \cdot \vec{v}_1)^2 - \frac{259}{2} \hat{n} \cdot \vec{S}_1 \hat{n} \cdot \vec{S}_2 \hat{n} \cdot \vec{v}_2 \hat{n} \cdot \vec{v}_1 + \frac{81}{2} \hat{n} \cdot \vec{v}_2 \vec{S}_1 \cdot \vec{S}_2 \hat{n} \cdot \vec{v}_1 + 49 \hat{n} \cdot \vec{S}_2 \right. \\ & \vec{S}_1 \cdot \vec{v}_1 \hat{n} \cdot \vec{v}_1 + \frac{53}{2} \hat{n} \cdot \vec{S}_2 \vec{S}_1 \cdot \vec{v}_2 \hat{n} \cdot \vec{v}_1 + 9 \hat{n} \cdot \vec{S}_1 \vec{S}_2 \cdot \vec{v}_1 \hat{n} \cdot \vec{v}_1 + \frac{53}{2} \hat{n} \cdot \vec{S}_1 \vec{S}_2 \cdot \vec{v}_2 \hat{n} \cdot \vec{v}_1 + 10 \hat{n} \times \vec{S}_1 \cdot \vec{v}_1 \hat{n} \times \vec{S}_2 \cdot \vec{v}_1 + \\ & 2 \hat{n} \times \vec{S}_1 \cdot \vec{v}_2 \hat{n} \times \vec{S}_2 \cdot \vec{v}_1 + \frac{1}{2} \hat{n} \cdot \vec{S}_2 \hat{n} \cdot \vec{v}_2 \vec{S}_1 \cdot \vec{v}_1 + \frac{37}{2} \hat{n} \cdot \vec{S}_1 \hat{n} \cdot \vec{v}_2 \vec{S}_2 \cdot \vec{v}_1 - 11 \vec{S}_1 \cdot \vec{v}_1 \vec{S}_2 \cdot \vec{v}_1 - \frac{9}{2} \vec{S}_1 \cdot \vec{v}_2 \vec{S}_2 \cdot \vec{v}_1 - \\ & \frac{1}{2} \vec{S}_1 \cdot \vec{v}_1 \vec{S}_2 \cdot \vec{v}_2 + \frac{1}{2} \hat{n} \cdot \vec{S}_1 \hat{n} \cdot \vec{S}_2 \vec{v}_1 \cdot \vec{v}_1 + \frac{27}{2} \vec{S}_1 \cdot \vec{S}_2 \vec{v}_1 \cdot \vec{v}_1 + \frac{53}{2} \hat{n} \cdot \vec{S}_1 \hat{n} \cdot \vec{S}_2 \vec{v}_1 \cdot \vec{v}_2 - \frac{33}{2} \vec{S}_1 \cdot \vec{S}_2 \vec{v}_1 \cdot \vec{v}_2 \Big) + \\ & \pi^2 \Bigg( \frac{1}{r^4} \left( -\frac{15}{2} \hat{n} \cdot \vec{S}_2 \hat{n} \cdot \vec{S}_1 \hat{n} \cdot \vec{v}_1 + \frac{75}{8} \hat{n} \cdot \vec{S}_1 \hat{n} \cdot \vec{S}_2 \hat{n} \cdot \vec{v}_1 - \frac{15}{8} \vec{S}_1 \cdot \vec{S}_2 \hat{n} \cdot \vec{v}_1 + \frac{3}{2} \vec{S}_1 \cdot \vec{S}_2 \hat{n} \cdot \vec{v}_1 - \right. \\ & \frac{15}{8} \hat{n} \cdot \vec{S}_2 \vec{S}_1 \cdot \vec{v}_1 + \frac{3}{2} \hat{n} \cdot \vec{S}_1 \vec{S}_2 \cdot \vec{v}_1 + \frac{3}{2} \hat{n} \cdot \vec{S}_2 \vec{S}_1 \cdot \vec{v}_1 - \frac{15}{8} \hat{n} \cdot \vec{S}_1 \vec{S}_2 \cdot \vec{v}_1 \Big) + \frac{1}{r^5} \\ & \left( -\frac{105}{2} \hat{n} \cdot \vec{S}_1 \hat{n} \cdot \vec{S}_2 (\hat{n} \cdot \vec{v}_1)^2 + \frac{15}{2} \vec{S}_1 \cdot \vec{S}_2 (\hat{n} \cdot \vec{v}_1)^2 - \frac{315}{16} \hat{n} \cdot \vec{S}_1 \hat{n} \cdot \vec{S}_2 \hat{n} \cdot \vec{v}_2 \hat{n} \cdot \vec{v}_1 + \frac{45}{16} \hat{n} \cdot \vec{v}_2 \vec{S}_1 \cdot \vec{S}_2 \hat{n} \cdot \vec{v}_1 + \right. \\ & 15 \hat{n} \cdot \vec{S}_2 \vec{S}_1 \cdot \vec{v}_1 \hat{n} \cdot \vec{v}_1 + \frac{45}{16} \hat{n} \cdot \vec{S}_2 \vec{S}_1 \cdot \vec{v}_2 \hat{n} \cdot \vec{v}_1 + 15 \hat{n} \cdot \vec{S}_1 \vec{S}_2 \cdot \vec{v}_1 \hat{n} \cdot \vec{v}_1 + \frac{45}{16} \hat{n} \cdot \vec{S}_1 \vec{S}_2 \cdot \vec{v}_2 \hat{n} \cdot \vec{v}_1 + \\ & \frac{45}{16} \hat{n} \cdot \vec{S}_2 \hat{n} \cdot \vec{v}_2 \vec{S}_1 \cdot \vec{v}_1 + \frac{45}{16} \hat{n} \cdot \vec{S}_1 \hat{n} \cdot \vec{v}_2 \vec{S}_2 \cdot \vec{v}_1 - 3 \vec{S}_1 \cdot \vec{v}_1 \vec{S}_2 \cdot \vec{v}_1 - \frac{9}{16} \vec{S}_1 \cdot \vec{v}_2 \vec{S}_2 \cdot \vec{v}_1 - \frac{9}{16} \vec{S}_1 \cdot \vec{v}_1 \vec{S}_2 \cdot \vec{v}_2 + \\ & \left. \left. \frac{15}{2} \hat{n} \cdot \vec{S}_1 \hat{n} \cdot \vec{S}_2 \vec{v}_1 \cdot \vec{v}_1 - \frac{3}{2} \vec{S}_1 \cdot \vec{S}_2 \vec{v}_1 \cdot \vec{v}_1 + \frac{45}{16} \hat{n} \cdot \vec{S}_1 \hat{n} \cdot \vec{S}_2 \vec{v}_1 \cdot \vec{v}_2 - \frac{9}{16} \vec{S}_1 \cdot \vec{S}_2 \vec{v}_1 \cdot \vec{v}_2 \right) \right) \Bigg) m_1 m_2 \Big\} \end{aligned}$$

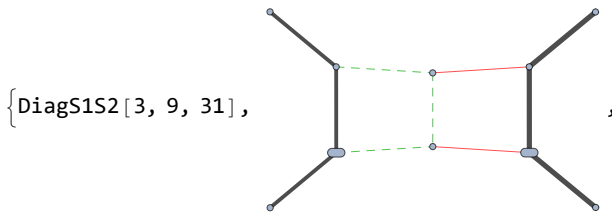

$$\frac{G^3 m_1 m_2 \left( 8 \vec{S}_1 \cdot \vec{S}_2 \hat{n} \cdot \vec{v}_1 \hat{n} \cdot \vec{v}_2 - 8 \hat{n} \cdot \vec{S}_1 \hat{n} \cdot \vec{v}_2 \vec{S}_2 \cdot \vec{v}_1 - 8 \vec{S}_1 \cdot \vec{S}_2 \vec{v}_1 \cdot \vec{v}_2 + 8 \vec{S}_1 \cdot \vec{v}_2 \vec{S}_2 \cdot \vec{v}_1 \right)}{r^5} \Big\}$$

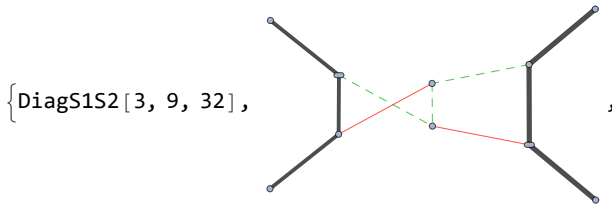

$$\frac{G^3 m_1 m_2 \left( -8 \vec{S}_1 \cdot \vec{S}_2 (\hat{n} \cdot \vec{v}_1)^2 + 8 \hat{n} \cdot \vec{S}_1 \hat{n} \cdot \vec{v}_1 \vec{S}_2 \cdot \vec{v}_1 - 8 \vec{S}_1 \cdot \vec{v}_1 \vec{S}_2 \cdot \vec{v}_1 + 8 \vec{S}_1 \cdot \vec{S}_2 \vec{v}_1 \cdot \vec{v}_1 \right)}{r^5} \Big\}$$

{DiagS1S2 [3, 9, 33],

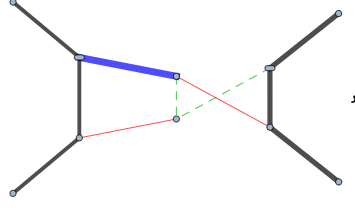

,

$$G^3 m_1 m_2 \left\{ \frac{1}{r^5} \left( 5 \hat{n} \times \vec{S}_1 \cdot \vec{v}_2 \hat{n} \times \vec{S}_2 \cdot \vec{v}_1 - 5 \hat{n} \times \vec{S}_1 \cdot \vec{v}_1 \hat{n} \times \vec{S}_2 \cdot \vec{v}_2 - 4 \hat{n} \times \vec{S}_1 \cdot \vec{v}_2 \hat{n} \times \vec{S}_2 \cdot \vec{v}_2 + \frac{149}{2} \hat{n} \cdot \vec{S}_1 \hat{n} \cdot \vec{S}_2 (\hat{n} \cdot \vec{v}_2)^2 - \right. \right. \\ \left. \frac{51}{2} \vec{S}_1 \cdot \vec{S}_2 (\hat{n} \cdot \vec{v}_2)^2 - \frac{211}{2} \hat{n} \cdot \vec{S}_1 \hat{n} \cdot \vec{S}_2 \hat{n} \cdot \vec{v}_1 \hat{n} \cdot \vec{v}_2 + \frac{89}{2} \vec{S}_1 \cdot \vec{S}_2 \hat{n} \cdot \vec{v}_1 \hat{n} \cdot \vec{v}_2 + \frac{35}{2} \hat{n} \cdot \vec{S}_2 \hat{n} \cdot \vec{v}_2 \vec{S}_1 \cdot \vec{v}_1 - \right. \\ \left. 5 \hat{n} \cdot \vec{S}_2 \hat{n} \cdot \vec{v}_2 \vec{S}_1 \cdot \vec{v}_2 + \frac{23}{2} \hat{n} \cdot \vec{S}_1 \hat{n} \cdot \vec{v}_2 \vec{S}_2 \cdot \vec{v}_1 - 21 \hat{n} \cdot \vec{S}_1 \hat{n} \cdot \vec{v}_2 \vec{S}_2 \cdot \vec{v}_2 - \frac{5}{2} \hat{n} \cdot \vec{S}_2 \hat{n} \cdot \vec{v}_1 \vec{S}_1 \cdot \vec{v}_2 + \right. \\ \left. \frac{23}{2} \hat{n} \cdot \vec{S}_1 \hat{n} \cdot \vec{v}_1 \vec{S}_2 \cdot \vec{v}_2 + \frac{25}{2} \vec{v}_1 \cdot \vec{v}_2 \hat{n} \cdot \vec{S}_1 \hat{n} \cdot \vec{S}_2 - \frac{19}{2} \vec{v}_2 \cdot \vec{v}_2 \hat{n} \cdot \vec{S}_1 \hat{n} \cdot \vec{S}_2 + \frac{1}{2} \vec{S}_1 \cdot \vec{v}_2 \vec{S}_2 \cdot \vec{v}_1 - \frac{3}{2} \vec{S}_1 \cdot \vec{v}_1 \vec{S}_2 \cdot \vec{v}_2 - \right. \\ \left. \vec{S}_1 \cdot \vec{v}_2 \vec{S}_2 \cdot \vec{v}_2 - \frac{17}{2} \vec{S}_1 \cdot \vec{S}_2 \vec{v}_1 \cdot \vec{v}_2 + \frac{15}{2} \vec{S}_1 \cdot \vec{S}_2 \vec{v}_2 \cdot \vec{v}_2 \right) + \frac{18 \hat{n} \cdot \vec{S}_1 \hat{n} \cdot \vec{S}_2 \hat{n} \cdot \vec{v}_2 - 6 \vec{S}_1 \cdot \vec{S}_2 \hat{n} \cdot \vec{v}_2 - 4 \hat{n} \cdot \vec{S}_1 \vec{S}_2 \cdot \vec{v}_2}{r^4} + \\ \left. \frac{\pi^2 \left( \frac{15}{8} \hat{n} \cdot \vec{S}_1 \hat{n} \cdot \vec{S}_2 \hat{n} \cdot \vec{v}_2 - \frac{3}{8} \vec{S}_1 \cdot \vec{S}_2 \hat{n} \cdot \vec{v}_2 - \frac{3}{8} \hat{n} \cdot \vec{S}_2 \vec{S}_1 \cdot \vec{v}_2 - \frac{3}{8} \hat{n} \cdot \vec{S}_1 \vec{S}_2 \cdot \vec{v}_2 \right)}{r^4} \right\}$$

{DiagS1S2 [3, 9, 34],

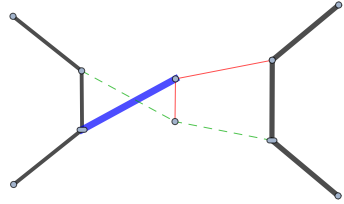

,  $\frac{1}{r^5}$

$$G^3 m_1 m_2 \left\{ -16 \hat{n} \times \vec{S}_1 \cdot \vec{v}_2 \hat{n} \times \vec{S}_2 \cdot \vec{v}_2 - 21 \hat{n} \cdot \vec{S}_1 \hat{n} \cdot \vec{S}_2 (\hat{n} \cdot \vec{v}_2)^2 + \vec{S}_1 \cdot \vec{S}_2 (\hat{n} \cdot \vec{v}_2)^2 + \right. \\ \left. 10 \hat{n} \cdot \vec{S}_2 \hat{n} \cdot \vec{v}_2 \vec{S}_1 \cdot \vec{v}_2 + 10 \hat{n} \cdot \vec{S}_1 \hat{n} \cdot \vec{v}_2 \vec{S}_2 \cdot \vec{v}_2 + \vec{v}_2 \cdot \vec{v}_2 \hat{n} \cdot \vec{S}_1 \hat{n} \cdot \vec{S}_2 - 6 \vec{S}_1 \cdot \vec{v}_2 \vec{S}_2 \cdot \vec{v}_2 + 5 \vec{S}_1 \cdot \vec{S}_2 \vec{v}_2 \cdot \vec{v}_2 \right\}$$

{DiagS1S2 [3, 9, 35],

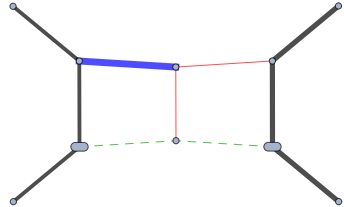

,

$$G^3 m_1 m_2 \left\{ \frac{1}{r^5} \left( -2 \hat{n} \times \vec{S}_1 \cdot \vec{v}_2 \hat{n} \times \vec{S}_2 \cdot \vec{v}_2 - 2 \hat{n} \cdot \vec{S}_1 \hat{n} \cdot \vec{S}_2 (\hat{n} \cdot \vec{v}_2)^2 - 8 \vec{S}_1 \cdot \vec{S}_2 (\hat{n} \cdot \vec{v}_2)^2 + 12 \hat{n} \cdot \vec{S}_1 \hat{n} \cdot \vec{v}_2 \vec{S}_2 \cdot \vec{v}_2 - \right. \right. \\ \left. 4 \vec{v}_2 \cdot \vec{v}_2 \hat{n} \cdot \vec{S}_1 \hat{n} \cdot \vec{S}_2 - 2 \vec{S}_1 \cdot \vec{v}_2 \vec{S}_2 \cdot \vec{v}_2 + 4 \vec{S}_1 \cdot \vec{S}_2 \vec{v}_2 \cdot \vec{v}_2 \right) + \frac{1}{r^5} \pi^2 \left( \frac{105}{32} \hat{n} \cdot \vec{S}_1 \hat{n} \cdot \vec{S}_2 (\hat{n} \cdot \vec{v}_2)^2 - \frac{15}{32} \vec{S}_1 \cdot \vec{S}_2 (\hat{n} \cdot \vec{v}_2)^2 - \right. \\ \left. \frac{15}{16} \hat{n} \cdot \vec{S}_2 \hat{n} \cdot \vec{v}_2 \vec{S}_1 \cdot \vec{v}_2 - \frac{15}{16} \hat{n} \cdot \vec{S}_1 \hat{n} \cdot \vec{v}_2 \vec{S}_2 \cdot \vec{v}_2 - \frac{15}{32} \vec{v}_2 \cdot \vec{v}_2 \hat{n} \cdot \vec{S}_1 \hat{n} \cdot \vec{S}_2 + \frac{3}{16} \vec{S}_1 \cdot \vec{v}_2 \vec{S}_2 \cdot \vec{v}_2 + \frac{3}{32} \vec{S}_1 \cdot \vec{S}_2 \vec{v}_2 \cdot \vec{v}_2 \right) \right\}$$

{DiagS1S2 [3, 9, 36],

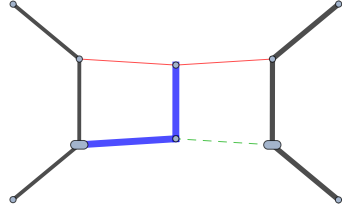

,

$$\begin{aligned}
 & G^3 \left( \frac{1}{r^4} \left( -29 \hat{n} \cdot \vec{a}_2 \hat{n} \cdot \vec{S}_1 \hat{n} \cdot \vec{S}_2 - 24 \hat{n} \cdot \vec{S}_1 \hat{n} \cdot \vec{v}_2 \hat{n} \cdot \vec{S}_2 + 17 \vec{S}_1 \cdot \vec{v}_2 \hat{n} \cdot \vec{S}_2 + 19 \vec{S}_1 \cdot \vec{a}_2 \hat{n} \cdot \vec{S}_2 - 29 \hat{n} \cdot \vec{S}_2 \hat{n} \cdot \vec{S}_1 \hat{n} \cdot \vec{v}_2 + \right. \right. \\
 & \quad \left. \hat{n} \cdot \vec{v}_2 \vec{S}_1 \cdot \vec{S}_2 + 2 \hat{n} \cdot \vec{S}_1 \vec{S}_2 \cdot \vec{v}_2 + 4 \hat{n} \cdot \vec{v}_2 \vec{S}_1 \cdot \vec{S}_2 + 4 \hat{n} \cdot \vec{a}_2 \vec{S}_1 \cdot \vec{S}_2 + 19 \hat{n} \cdot \vec{S}_2 \vec{S}_1 \cdot \vec{v}_2 + 2 \hat{n} \cdot \vec{S}_1 \vec{S}_2 \cdot \vec{a}_2 + 2 \hat{n} \cdot \vec{S}_1 \vec{S}_2 \cdot \vec{v}_2 \right) + \\
 & \quad \frac{1}{r^5} \left( -\frac{2571}{8} \hat{n} \cdot \vec{S}_1 \hat{n} \cdot \vec{S}_2 (\hat{n} \cdot \vec{v}_2)^2 + \frac{325}{8} \vec{S}_1 \cdot \vec{S}_2 (\hat{n} \cdot \vec{v}_2)^2 + \frac{2215}{8} \hat{n} \cdot \vec{S}_1 \hat{n} \cdot \vec{S}_2 \hat{n} \cdot \vec{v}_1 \hat{n} \cdot \vec{v}_2 - \right. \\
 & \quad \frac{189}{8} \hat{n} \cdot \vec{v}_1 \vec{S}_1 \cdot \vec{S}_2 \hat{n} \cdot \vec{v}_2 - \frac{273}{8} \hat{n} \cdot \vec{S}_2 \vec{S}_1 \cdot \vec{v}_1 \hat{n} \cdot \vec{v}_2 + \frac{505}{4} \hat{n} \cdot \vec{S}_2 \vec{S}_1 \cdot \vec{v}_2 \hat{n} \cdot \vec{v}_2 - \frac{301}{8} \hat{n} \cdot \vec{S}_1 \vec{S}_2 \cdot \vec{v}_1 \hat{n} \cdot \vec{v}_2 + \\
 & \quad \frac{309}{4} \hat{n} \cdot \vec{S}_1 \vec{S}_2 \cdot \vec{v}_2 \hat{n} \cdot \vec{v}_2 + 9 \hat{n} \times \vec{S}_1 \cdot \vec{v}_2 \hat{n} \times \vec{S}_2 \cdot \vec{v}_1 - 32 \hat{n} \times \vec{S}_1 \cdot \vec{v}_1 \hat{n} \times \vec{S}_2 \cdot \vec{v}_2 + 23 \hat{n} \times \vec{S}_1 \cdot \vec{v}_2 \hat{n} \times \vec{S}_2 \cdot \vec{v}_2 - \\
 & \quad \frac{633}{8} \hat{n} \cdot \vec{S}_2 \hat{n} \cdot \vec{v}_1 \vec{S}_1 \cdot \vec{v}_2 + \frac{105}{8} \vec{S}_1 \cdot \vec{v}_2 \vec{S}_2 \cdot \vec{v}_1 - \frac{273}{8} \hat{n} \cdot \vec{S}_1 \hat{n} \cdot \vec{v}_1 \vec{S}_2 \cdot \vec{v}_2 + \frac{69}{8} \vec{S}_1 \cdot \vec{v}_1 \vec{S}_2 \cdot \vec{v}_2 - \frac{81}{4} \vec{S}_1 \cdot \vec{v}_2 \vec{S}_2 \cdot \vec{v}_2 - \\
 & \quad \left. \frac{345}{8} \hat{n} \cdot \vec{S}_1 \hat{n} \cdot \vec{S}_2 \vec{v}_1 \cdot \vec{v}_2 + \frac{33}{8} \vec{S}_1 \cdot \vec{S}_2 \vec{v}_1 \cdot \vec{v}_2 + \frac{413}{8} \hat{n} \cdot \vec{S}_1 \hat{n} \cdot \vec{S}_2 \vec{v}_2 \cdot \vec{v}_2 - \frac{89}{8} \vec{S}_1 \cdot \vec{S}_2 \vec{v}_2 \cdot \vec{v}_2 \right) + \\
 & \quad \pi^2 \left( \frac{1}{r^4} \left( \frac{15}{8} \hat{n} \cdot \vec{a}_2 \hat{n} \cdot \vec{S}_1 \hat{n} \cdot \vec{S}_2 + \frac{15}{8} \hat{n} \cdot \vec{S}_1 \hat{n} \cdot \vec{v}_2 \hat{n} \cdot \vec{S}_2 - \frac{3}{8} \vec{S}_1 \cdot \vec{v}_2 \hat{n} \cdot \vec{S}_2 - \frac{3}{8} \vec{S}_1 \cdot \vec{a}_2 \hat{n} \cdot \vec{S}_2 + \right. \right. \\
 & \quad \frac{15}{8} \hat{n} \cdot \vec{S}_2 \hat{n} \cdot \vec{S}_1 \hat{n} \cdot \vec{v}_2 - \frac{3}{8} \hat{n} \cdot \vec{v}_2 \vec{S}_1 \cdot \vec{S}_2 - \frac{3}{8} \hat{n} \cdot \vec{S}_1 \vec{S}_2 \cdot \vec{v}_2 - \frac{3}{8} \hat{n} \cdot \vec{v}_2 \vec{S}_1 \cdot \vec{S}_2 - \\
 & \quad \left. \frac{3}{8} \hat{n} \cdot \vec{a}_2 \vec{S}_1 \cdot \vec{S}_2 - \frac{3}{8} \hat{n} \cdot \vec{S}_2 \vec{S}_1 \cdot \vec{v}_2 - \frac{3}{8} \hat{n} \cdot \vec{S}_1 \vec{S}_2 \cdot \vec{a}_2 - \frac{3}{8} \hat{n} \cdot \vec{S}_1 \vec{S}_2 \cdot \vec{v}_2 \right) + \frac{1}{r^5} \\
 & \quad \left( \frac{3255}{128} \hat{n} \cdot \vec{S}_1 \hat{n} \cdot \vec{S}_2 (\hat{n} \cdot \vec{v}_2)^2 - \frac{465}{128} \vec{S}_1 \cdot \vec{S}_2 (\hat{n} \cdot \vec{v}_2)^2 - \frac{2835}{128} \hat{n} \cdot \vec{S}_1 \hat{n} \cdot \vec{S}_2 \hat{n} \cdot \vec{v}_1 \hat{n} \cdot \vec{v}_2 + \frac{405}{128} \hat{n} \cdot \vec{v}_1 \vec{S}_1 \cdot \vec{S}_2 \hat{n} \cdot \vec{v}_2 + \right. \\
 & \quad \frac{405}{128} \hat{n} \cdot \vec{S}_2 \vec{S}_1 \cdot \vec{v}_1 \hat{n} \cdot \vec{v}_2 - \frac{465}{64} \hat{n} \cdot \vec{S}_2 \vec{S}_1 \cdot \vec{v}_2 \hat{n} \cdot \vec{v}_2 + \frac{405}{128} \hat{n} \cdot \vec{S}_1 \vec{S}_2 \cdot \vec{v}_1 \hat{n} \cdot \vec{v}_2 - \frac{465}{64} \hat{n} \cdot \vec{S}_1 \vec{S}_2 \cdot \vec{v}_2 \hat{n} \cdot \vec{v}_2 + \\
 & \quad \frac{405}{128} \hat{n} \cdot \vec{S}_2 \hat{n} \cdot \vec{v}_1 \vec{S}_1 \cdot \vec{v}_2 - \frac{81}{128} \vec{S}_1 \cdot \vec{v}_2 \vec{S}_2 \cdot \vec{v}_1 + \frac{405}{128} \hat{n} \cdot \vec{S}_1 \hat{n} \cdot \vec{v}_1 \vec{S}_2 \cdot \vec{v}_2 - \frac{81}{128} \vec{S}_1 \cdot \vec{v}_1 \vec{S}_2 \cdot \vec{v}_2 + \frac{93}{64} \vec{S}_1 \cdot \vec{v}_2 \vec{S}_2 \cdot \vec{v}_2 + \\
 & \quad \left. \left. \frac{405}{128} \hat{n} \cdot \vec{S}_1 \hat{n} \cdot \vec{S}_2 \vec{v}_1 \cdot \vec{v}_2 - \frac{81}{128} \vec{S}_1 \cdot \vec{S}_2 \vec{v}_1 \cdot \vec{v}_2 - \frac{465}{128} \hat{n} \cdot \vec{S}_1 \hat{n} \cdot \vec{S}_2 \vec{v}_2 \cdot \vec{v}_2 + \frac{93}{128} \vec{S}_1 \cdot \vec{S}_2 \vec{v}_2 \cdot \vec{v}_2 \right) \right) \Bigg\} m_1 m_2 \Bigg\}
 \end{aligned}$$

{DiagS1S2 [3, 9, 37],

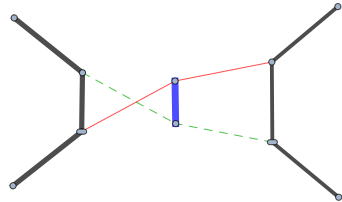

,

$$\frac{G^3 m_1 m_2 \left( -12 \hat{n} \times \vec{S}_1 \cdot \vec{v}_1 \hat{n} \times \vec{S}_2 \cdot \vec{v}_1 - 28 \vec{S}_1 \cdot \vec{S}_2 (\hat{n} \cdot \vec{v}_1)^2 + 28 \hat{n} \cdot \vec{S}_1 \hat{n} \cdot \vec{v}_1 \vec{S}_2 \cdot \vec{v}_1 - 48 \vec{S}_1 \cdot \vec{v}_1 \vec{S}_2 \cdot \vec{v}_1 + 48 \vec{S}_1 \cdot \vec{S}_2 \vec{v}_1 \cdot \vec{v}_1 \right)}{r^5}$$

{DiagS1S2 [3, 9, 38],

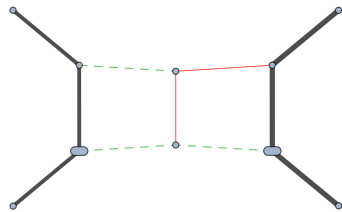

,

$$\begin{aligned}
& G^3 \left( \frac{1}{r^4} \left( -26 \hat{n} \cdot \vec{S}_2 \hat{n} \cdot \vec{S}_1 \hat{n} \cdot \vec{v}_2 - 26 \hat{n} \cdot \vec{S}_1 \hat{n} \cdot \vec{S}_2 \hat{n} \cdot \vec{v}_2 + 12 \vec{S}_1 \cdot \vec{S}_2 \hat{n} \cdot \vec{v}_2 + \right. \right. \\
& \quad \left. \left. 12 \vec{S}_1 \cdot \vec{S}_2 \hat{n} \cdot \vec{v}_2 - 2 \hat{n} \cdot \vec{S}_2 \vec{S}_1 \cdot \vec{v}_2 - 4 \hat{n} \cdot \vec{S}_1 \vec{S}_2 \cdot \vec{v}_2 - 2 \hat{n} \cdot \vec{S}_2 \vec{S}_1 \cdot \vec{v}_2 - 4 \hat{n} \cdot \vec{S}_1 \vec{S}_2 \cdot \vec{v}_2 \right) + \frac{1}{r^5} \right. \\
& \quad \left( -150 \hat{n} \cdot \vec{S}_1 \hat{n} \cdot \vec{S}_2 (\hat{n} \cdot \vec{v}_2)^2 + 38 \vec{S}_1 \cdot \vec{S}_2 (\hat{n} \cdot \vec{v}_2)^2 + 154 \hat{n} \cdot \vec{S}_1 \hat{n} \cdot \vec{S}_2 \hat{n} \cdot \vec{v}_1 \hat{n} \cdot \vec{v}_2 - 22 \hat{n} \cdot \vec{v}_1 \vec{S}_1 \cdot \vec{S}_2 \hat{n} \cdot \vec{v}_2 - \right. \\
& \quad 31 \hat{n} \cdot \vec{S}_2 \vec{S}_1 \cdot \vec{v}_1 \hat{n} \cdot \vec{v}_2 + 28 \hat{n} \cdot \vec{S}_2 \vec{S}_1 \cdot \vec{v}_2 \hat{n} \cdot \vec{v}_2 - 45 \hat{n} \cdot \vec{S}_1 \vec{S}_2 \cdot \vec{v}_1 \hat{n} \cdot \vec{v}_2 + 18 \hat{n} \cdot \vec{S}_1 \vec{S}_2 \cdot \vec{v}_2 \hat{n} \cdot \vec{v}_2 + \\
& \quad 5 \hat{n} \times \vec{S}_1 \cdot \vec{v}_2 \hat{n} \times \vec{S}_2 \cdot \vec{v}_1 + 5 \hat{n} \times \vec{S}_1 \cdot \vec{v}_1 \hat{n} \times \vec{S}_2 \cdot \vec{v}_2 - 6 \hat{n} \times \vec{S}_1 \cdot \vec{v}_2 \hat{n} \times \vec{S}_2 \cdot \vec{v}_2 + 3 \hat{n} \cdot \vec{S}_2 \hat{n} \cdot \vec{v}_1 \vec{S}_1 \cdot \vec{v}_2 + 3 \vec{S}_1 \cdot \vec{v}_2 \vec{S}_2 \cdot \vec{v}_1 + \\
& \quad \left. 3 \hat{n} \cdot \vec{S}_1 \hat{n} \cdot \vec{v}_1 \vec{S}_2 \cdot \vec{v}_2 + \vec{S}_1 \cdot \vec{v}_1 \vec{S}_2 \cdot \vec{v}_2 + 8 \hat{n} \cdot \vec{S}_1 \hat{n} \cdot \vec{S}_2 \vec{v}_1 \cdot \vec{v}_2 - 10 \vec{S}_1 \cdot \vec{S}_2 \vec{v}_1 \cdot \vec{v}_2 + 2 \vec{S}_1 \cdot \vec{S}_2 \vec{v}_2 \cdot \vec{v}_2 \right) + \\
& \quad \pi^2 \left( \frac{1}{r^4} \left( -\frac{15}{8} \hat{n} \cdot \vec{S}_2 \hat{n} \cdot \vec{S}_1 \hat{n} \cdot \vec{v}_2 - \frac{15}{8} \hat{n} \cdot \vec{S}_1 \hat{n} \cdot \vec{S}_2 \hat{n} \cdot \vec{v}_2 + \frac{3}{8} \vec{S}_1 \cdot \vec{S}_2 \hat{n} \cdot \vec{v}_2 + \frac{3}{8} \vec{S}_1 \cdot \vec{S}_2 \hat{n} \cdot \vec{v}_2 + \right. \right. \\
& \quad \left. \left. \frac{3}{8} \hat{n} \cdot \vec{S}_2 \vec{S}_1 \cdot \vec{v}_2 + \frac{3}{8} \hat{n} \cdot \vec{S}_1 \vec{S}_2 \cdot \vec{v}_2 + \frac{3}{8} \hat{n} \cdot \vec{S}_2 \vec{S}_1 \cdot \vec{v}_2 + \frac{3}{8} \hat{n} \cdot \vec{S}_1 \vec{S}_2 \cdot \vec{v}_2 \right) + \frac{1}{r^5} \right. \\
& \quad \left( -\frac{315}{32} \hat{n} \cdot \vec{S}_1 \hat{n} \cdot \vec{S}_2 (\hat{n} \cdot \vec{v}_2)^2 + \frac{45}{32} \vec{S}_1 \cdot \vec{S}_2 (\hat{n} \cdot \vec{v}_2)^2 + \frac{105}{32} \hat{n} \cdot \vec{S}_1 \hat{n} \cdot \vec{S}_2 \hat{n} \cdot \vec{v}_1 \hat{n} \cdot \vec{v}_2 - \frac{15}{32} \hat{n} \cdot \vec{v}_1 \vec{S}_1 \cdot \vec{S}_2 \hat{n} \cdot \vec{v}_2 - \right. \\
& \quad \frac{15}{32} \hat{n} \cdot \vec{S}_2 \vec{S}_1 \cdot \vec{v}_1 \hat{n} \cdot \vec{v}_2 + \frac{45}{16} \hat{n} \cdot \vec{S}_2 \vec{S}_1 \cdot \vec{v}_2 \hat{n} \cdot \vec{v}_2 - \frac{15}{32} \hat{n} \cdot \vec{S}_1 \vec{S}_2 \cdot \vec{v}_1 \hat{n} \cdot \vec{v}_2 + \frac{45}{16} \hat{n} \cdot \vec{S}_1 \vec{S}_2 \cdot \vec{v}_2 \hat{n} \cdot \vec{v}_2 - \\
& \quad \frac{15}{32} \hat{n} \cdot \vec{S}_2 \hat{n} \cdot \vec{v}_1 \vec{S}_1 \cdot \vec{v}_2 + \frac{3}{32} \vec{S}_1 \cdot \vec{v}_2 \vec{S}_2 \cdot \vec{v}_1 - \frac{15}{32} \hat{n} \cdot \vec{S}_1 \hat{n} \cdot \vec{v}_1 \vec{S}_2 \cdot \vec{v}_2 + \frac{3}{32} \vec{S}_1 \cdot \vec{v}_1 \vec{S}_2 \cdot \vec{v}_2 - \frac{9}{16} \vec{S}_1 \cdot \vec{v}_2 \vec{S}_2 \cdot \vec{v}_2 - \\
& \quad \left. \left. \frac{15}{32} \hat{n} \cdot \vec{S}_1 \hat{n} \cdot \vec{S}_2 \vec{v}_1 \cdot \vec{v}_2 + \frac{3}{32} \vec{S}_1 \cdot \vec{S}_2 \vec{v}_1 \cdot \vec{v}_2 + \frac{45}{32} \hat{n} \cdot \vec{S}_1 \hat{n} \cdot \vec{S}_2 \vec{v}_2 \cdot \vec{v}_2 - \frac{9}{32} \vec{S}_1 \cdot \vec{S}_2 \vec{v}_2 \cdot \vec{v}_2 \right) \right) \Bigg) m_1 m_2 \Bigg\}
\end{aligned}$$

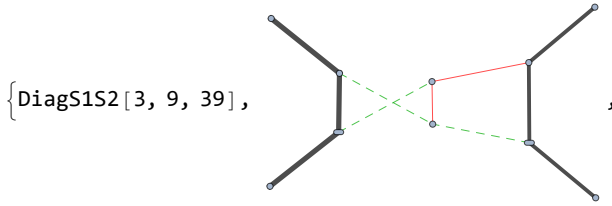

$$\begin{aligned}
& G^3 m_1 m_2 \left( \frac{-10 \hat{n} \cdot \vec{a}_1 \hat{n} \cdot \vec{S}_1 \hat{n} \cdot \vec{S}_2 + 6 \vec{S}_1 \cdot \vec{a}_1 \hat{n} \cdot \vec{S}_2 + 4 \vec{S}_1 \cdot \vec{S}_2 \hat{n} \cdot \vec{a}_1 - 10 \hat{n} \cdot \vec{S}_2 \hat{n} \cdot \vec{S}_1 \hat{n} \cdot \vec{v}_1 + 4 \vec{S}_1 \cdot \vec{S}_2 \hat{n} \cdot \vec{v}_1 + 6 \hat{n} \cdot \vec{S}_2 \vec{S}_1 \cdot \vec{v}_1}{r^4} + \right. \\
& \quad \frac{1}{r^5} \left( -4 \hat{n} \times \vec{S}_1 \cdot \vec{v}_1 \hat{n} \times \vec{S}_2 \cdot \vec{v}_1 + 16 \hat{n} \times \vec{S}_1 \cdot \vec{v}_2 \hat{n} \times \vec{S}_2 \cdot \vec{v}_1 + 4 \hat{n} \times \vec{S}_1 \cdot \vec{v}_1 \hat{n} \times \vec{S}_2 \cdot \vec{v}_2 + \right. \\
& \quad 39 \hat{n} \cdot \vec{S}_1 \hat{n} \cdot \vec{S}_2 (\hat{n} \cdot \vec{v}_1)^2 - 17 \vec{S}_1 \cdot \vec{S}_2 (\hat{n} \cdot \vec{v}_1)^2 - 18 \hat{n} \cdot \vec{S}_1 \hat{n} \cdot \vec{S}_2 \hat{n} \cdot \vec{v}_2 \hat{n} \cdot \vec{v}_1 + 16 \vec{S}_1 \cdot \vec{S}_2 \hat{n} \cdot \vec{v}_2 \hat{n} \cdot \vec{v}_1 - \\
& \quad 22 \hat{n} \cdot \vec{S}_2 \hat{n} \cdot \vec{v}_1 \vec{S}_1 \cdot \vec{v}_1 + 10 \hat{n} \cdot \vec{S}_2 \hat{n} \cdot \vec{v}_1 \vec{S}_1 \cdot \vec{v}_2 - 10 \hat{n} \cdot \vec{S}_1 \hat{n} \cdot \vec{v}_1 \vec{S}_2 \cdot \vec{v}_2 + 2 \hat{n} \cdot \vec{S}_2 \hat{n} \cdot \vec{v}_2 \vec{S}_1 \cdot \vec{v}_1 - \\
& \quad \left. \left. 7 \vec{v}_1 \cdot \vec{v}_1 \hat{n} \cdot \vec{S}_1 \hat{n} \cdot \vec{S}_2 + 6 \vec{v}_1 \cdot \vec{v}_2 \hat{n} \cdot \vec{S}_1 \hat{n} \cdot \vec{S}_2 + 6 \vec{S}_1 \cdot \vec{v}_1 \vec{S}_2 \cdot \vec{v}_2 + 7 \vec{S}_1 \cdot \vec{S}_2 \vec{v}_1 \cdot \vec{v}_1 - 12 \vec{S}_1 \cdot \vec{S}_2 \vec{v}_1 \cdot \vec{v}_2 \right) \right) \Bigg\}
\end{aligned}$$

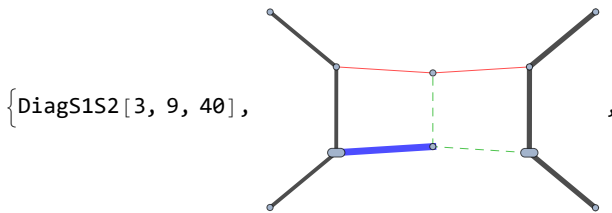

$$\begin{aligned}
& G^3 \left( \frac{1}{r^5} \left( -\frac{163}{8} \hat{n} \cdot \vec{S}_1 \hat{n} \cdot \vec{S}_2 (\hat{n} \cdot \vec{v}_2)^2 + \frac{29}{8} \vec{S}_1 \cdot \vec{S}_2 (\hat{n} \cdot \vec{v}_2)^2 - \frac{65}{8} \hat{n} \cdot \vec{S}_1 \hat{n} \cdot \vec{S}_2 \hat{n} \cdot \vec{v}_1 \hat{n} \cdot \vec{v}_2 + \right. \right. \\
& \quad \frac{19}{8} \hat{n} \cdot \vec{v}_1 \vec{S}_1 \cdot \vec{S}_2 \hat{n} \cdot \vec{v}_2 + \frac{19}{8} \hat{n} \cdot \vec{S}_2 \vec{S}_1 \cdot \vec{v}_1 \hat{n} \cdot \vec{v}_2 + \frac{25}{4} \hat{n} \cdot \vec{S}_2 \vec{S}_1 \cdot \vec{v}_2 \hat{n} \cdot \vec{v}_2 - \frac{9}{8} \hat{n} \cdot \vec{S}_1 \vec{S}_2 \cdot \vec{v}_1 \hat{n} \cdot \vec{v}_2 + \\
& \quad \left. \frac{21}{4} \hat{n} \cdot \vec{S}_1 \vec{S}_2 \cdot \vec{v}_2 \hat{n} \cdot \vec{v}_2 - \frac{7}{2} \hat{n} \times \vec{S}_1 \cdot \vec{v}_2 \hat{n} \times \vec{S}_2 \cdot \vec{v}_1 + \frac{17}{2} \hat{n} \times \vec{S}_1 \cdot \vec{v}_1 \hat{n} \times \vec{S}_2 \cdot \vec{v}_2 - 2 \hat{n} \times \vec{S}_1 \cdot \vec{v}_2 \hat{n} \times \vec{S}_2 \cdot \vec{v}_2 - \right.
\end{aligned}$$

$$\pi^2 \left( \frac{105}{128} \hat{n} \cdot \vec{S}_1 \hat{n} \cdot \vec{S}_2 (\hat{n} \cdot \vec{v}_2)^2 - \frac{15}{128} \vec{S}_1 \cdot \vec{S}_2 (\hat{n} \cdot \vec{v}_2)^2 + \frac{105}{128} \hat{n} \cdot \vec{S}_1 \hat{n} \cdot \vec{S}_2 \hat{n} \cdot \vec{v}_1 \hat{n} \cdot \vec{v}_2 - \frac{15}{128} \hat{n} \cdot \vec{v}_1 \vec{S}_1 \cdot \vec{S}_2 \hat{n} \cdot \vec{v}_2 - \frac{15}{128} \hat{n} \cdot \vec{S}_2 \vec{S}_1 \cdot \vec{v}_1 \hat{n} \cdot \vec{v}_2 - \frac{15}{64} \hat{n} \cdot \vec{S}_2 \vec{S}_1 \cdot \vec{v}_2 \hat{n} \cdot \vec{v}_2 - \frac{15}{128} \hat{n} \cdot \vec{S}_1 \vec{S}_2 \cdot \vec{v}_1 \hat{n} \cdot \vec{v}_2 - \frac{15}{64} \hat{n} \cdot \vec{S}_1 \vec{S}_2 \cdot \vec{v}_2 \hat{n} \cdot \vec{v}_2 - \frac{15}{128} \hat{n} \cdot \vec{S}_2 \hat{n} \cdot \vec{v}_1 \vec{S}_1 \cdot \vec{v}_2 + \frac{3}{128} \vec{S}_1 \cdot \vec{v}_2 \vec{S}_2 \cdot \vec{v}_1 - \frac{15}{128} \hat{n} \cdot \vec{S}_1 \hat{n} \cdot \vec{v}_1 \vec{S}_2 \cdot \vec{v}_2 + \frac{3}{128} \vec{S}_1 \cdot \vec{v}_1 \vec{S}_2 \cdot \vec{v}_2 + \frac{3}{64} \vec{S}_1 \cdot \vec{v}_2 \vec{S}_2 \cdot \vec{v}_2 - \frac{15}{128} \hat{n} \cdot \vec{S}_1 \hat{n} \cdot \vec{S}_2 \vec{v}_1 \cdot \vec{v}_2 + \frac{3}{128} \vec{S}_1 \cdot \vec{S}_2 \vec{v}_1 \cdot \vec{v}_2 - \frac{15}{128} \hat{n} \cdot \vec{S}_1 \hat{n} \cdot \vec{S}_2 \vec{v}_2 \cdot \vec{v}_2 + \frac{3}{128} \vec{S}_1 \cdot \vec{S}_2 \vec{v}_2 \cdot \vec{v}_2 \right) m_1 m_2 \}$$

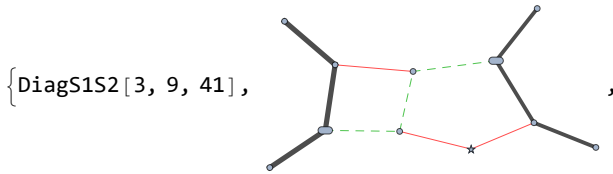

$$\begin{aligned} & \mathcal{G}^3 \left( \frac{1}{r^4} \left( -8 \hat{n} \cdot \vec{S}_2 \hat{n} \cdot \vec{S}_1 \hat{n} \cdot \vec{v}_2 - 8 \hat{n} \cdot \vec{S}_1 \hat{n} \cdot \vec{S}_2 \hat{n} \cdot \vec{v}_2 + 3 \vec{S}_1 \cdot \vec{S}_2 \hat{n} \cdot \vec{v}_2 + 3 \vec{S}_1 \cdot \vec{S}_2 \hat{n} \cdot \vec{v}_2 + \hat{n} \cdot \vec{S}_2 \vec{S}_1 \cdot \vec{v}_2 + \right. \right. \\ & \quad 2 \hat{n} \cdot \vec{S}_1 \vec{S}_2 \cdot \vec{v}_2 + \hat{n} \cdot \vec{S}_2 \vec{S}_1 \cdot \vec{v}_2 + 2 \hat{n} \cdot \vec{S}_1 \vec{S}_2 \cdot \vec{v}_2 \left. \right) + \frac{1}{r^5} \left( -36 \hat{n} \cdot \vec{S}_1 \hat{n} \cdot \vec{S}_2 (\hat{n} \cdot \vec{v}_2)^2 + 11 \vec{S}_1 \cdot \vec{S}_2 (\hat{n} \cdot \vec{v}_2)^2 + \right. \\ & \quad 56 \hat{n} \cdot \vec{S}_1 \hat{n} \cdot \vec{S}_2 \hat{n} \cdot \vec{v}_1 \hat{n} \cdot \vec{v}_2 - 15 \hat{n} \cdot \vec{v}_1 \vec{S}_1 \cdot \vec{S}_2 \hat{n} \cdot \vec{v}_2 - 8 \hat{n} \cdot \vec{S}_2 \vec{S}_1 \cdot \vec{v}_1 \hat{n} \cdot \vec{v}_2 + 7 \hat{n} \cdot \vec{S}_2 \vec{S}_1 \cdot \vec{v}_2 \hat{n} \cdot \vec{v}_2 - \\ & \quad 8 \hat{n} \cdot \vec{S}_1 \vec{S}_2 \cdot \vec{v}_1 \hat{n} \cdot \vec{v}_2 + 10 \hat{n} \cdot \vec{S}_1 \vec{S}_2 \cdot \vec{v}_2 \hat{n} \cdot \vec{v}_2 - 5 \hat{n} \cdot \vec{S}_2 \hat{n} \cdot \vec{v}_1 \vec{S}_1 \cdot \vec{v}_2 + \vec{S}_1 \cdot \vec{v}_2 \vec{S}_2 \cdot \vec{v}_1 - 10 \hat{n} \cdot \vec{S}_1 \hat{n} \cdot \vec{v}_1 \vec{S}_2 \cdot \vec{v}_2 + \\ & \quad 2 \vec{S}_1 \cdot \vec{v}_1 \vec{S}_2 \cdot \vec{v}_2 - \vec{S}_1 \cdot \vec{v}_2 \vec{S}_2 \cdot \vec{v}_2 - 8 \hat{n} \cdot \vec{S}_1 \hat{n} \cdot \vec{S}_2 \vec{v}_1 \cdot \vec{v}_2 + 3 \vec{S}_1 \cdot \vec{S}_2 \vec{v}_1 \cdot \vec{v}_2 + 2 \hat{n} \cdot \vec{S}_1 \hat{n} \cdot \vec{S}_2 \vec{v}_2 \cdot \vec{v}_2 - \vec{S}_1 \cdot \vec{S}_2 \vec{v}_2 \cdot \vec{v}_2 \left. \right) + \\ & \quad \pi^2 \left( \frac{1}{r^4} \left( \frac{15}{8} \hat{n} \cdot \vec{S}_2 \hat{n} \cdot \vec{S}_1 \hat{n} \cdot \vec{v}_2 + \frac{15}{8} \hat{n} \cdot \vec{S}_1 \hat{n} \cdot \vec{S}_2 \hat{n} \cdot \vec{v}_2 - \frac{3}{8} \vec{S}_1 \cdot \vec{S}_2 \hat{n} \cdot \vec{v}_2 - \frac{3}{8} \vec{S}_1 \cdot \vec{S}_2 \hat{n} \cdot \vec{v}_2 - \right. \right. \\ & \quad \left. \frac{3}{8} \hat{n} \cdot \vec{S}_2 \vec{S}_1 \cdot \vec{v}_2 - \frac{3}{8} \hat{n} \cdot \vec{S}_1 \vec{S}_2 \cdot \vec{v}_2 - \frac{3}{8} \hat{n} \cdot \vec{S}_2 \vec{S}_1 \cdot \vec{v}_2 - \frac{3}{8} \hat{n} \cdot \vec{S}_1 \vec{S}_2 \cdot \vec{v}_2 \right) + \frac{1}{r^5} \\ & \quad \left( \frac{1365}{128} \hat{n} \cdot \vec{S}_1 \hat{n} \cdot \vec{S}_2 (\hat{n} \cdot \vec{v}_2)^2 - \frac{195}{128} \vec{S}_1 \cdot \vec{S}_2 (\hat{n} \cdot \vec{v}_2)^2 - \frac{105}{8} \hat{n} \cdot \vec{S}_1 \hat{n} \cdot \vec{S}_2 \hat{n} \cdot \vec{v}_1 \hat{n} \cdot \vec{v}_2 + \frac{15}{8} \hat{n} \cdot \vec{v}_1 \vec{S}_1 \cdot \vec{S}_2 \hat{n} \cdot \vec{v}_2 + \right. \\ & \quad \frac{15}{8} \hat{n} \cdot \vec{S}_2 \vec{S}_1 \cdot \vec{v}_1 \hat{n} \cdot \vec{v}_2 - \frac{195}{64} \hat{n} \cdot \vec{S}_2 \vec{S}_1 \cdot \vec{v}_2 \hat{n} \cdot \vec{v}_2 + \frac{15}{8} \hat{n} \cdot \vec{S}_1 \vec{S}_2 \cdot \vec{v}_1 \hat{n} \cdot \vec{v}_2 - \frac{195}{64} \hat{n} \cdot \vec{S}_1 \vec{S}_2 \cdot \vec{v}_2 \hat{n} \cdot \vec{v}_2 + \\ & \quad \frac{15}{8} \hat{n} \cdot \vec{S}_2 \hat{n} \cdot \vec{v}_1 \vec{S}_1 \cdot \vec{v}_2 - \frac{3}{8} \vec{S}_1 \cdot \vec{v}_2 \vec{S}_2 \cdot \vec{v}_1 + \frac{15}{8} \hat{n} \cdot \vec{S}_1 \hat{n} \cdot \vec{v}_1 \vec{S}_2 \cdot \vec{v}_2 - \frac{3}{8} \vec{S}_1 \cdot \vec{v}_1 \vec{S}_2 \cdot \vec{v}_2 + \frac{39}{64} \vec{S}_1 \cdot \vec{v}_2 \vec{S}_2 \cdot \vec{v}_2 + \\ & \quad \left. \left. \frac{15}{8} \hat{n} \cdot \vec{S}_1 \hat{n} \cdot \vec{S}_2 \vec{v}_1 \cdot \vec{v}_2 - \frac{3}{8} \vec{S}_1 \cdot \vec{S}_2 \vec{v}_1 \cdot \vec{v}_2 - \frac{195}{128} \hat{n} \cdot \vec{S}_1 \hat{n} \cdot \vec{S}_2 \vec{v}_2 \cdot \vec{v}_2 + \frac{39}{128} \vec{S}_1 \cdot \vec{S}_2 \vec{v}_2 \cdot \vec{v}_2 \right) \right) \Bigg\} m_1 m_2 \Bigg\} \end{aligned}$$

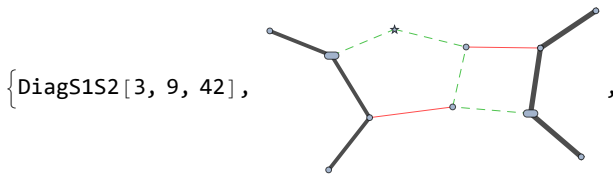

$$G^3 \left( \frac{2 \hat{n} \cdot \vec{S}_1 \hat{n} \cdot \vec{S}_2}{r^3} + \frac{1}{r^4} \left( -10 \hat{n} \cdot \vec{S}_2 \hat{n} \cdot \vec{S}_1 \hat{n} \cdot \vec{v}_1 + 15 \hat{n} \cdot \vec{S}_2 \hat{n} \cdot \vec{S}_1 \hat{n} \cdot \vec{v}_2 - 5 \hat{n} \cdot \vec{S}_1 \hat{n} \cdot \vec{S}_2 \hat{n} \cdot \vec{v}_2 + \right. \right. \\ \left. \left. 2 \hat{n} \cdot \vec{S}_2 \vec{S}_1 \cdot \vec{v}_2 + 2 \hat{n} \cdot \vec{S}_1 \vec{S}_2 \cdot \vec{v}_1 - 3 \hat{n} \cdot \vec{S}_1 \vec{S}_2 \cdot \vec{v}_2 + 2 \hat{n} \cdot \vec{S}_2 \vec{S}_1 \cdot \vec{v}_1 - 4 \hat{n} \cdot \vec{S}_2 \vec{S}_1 \cdot \vec{v}_2 + \hat{n} \cdot \vec{S}_1 \vec{S}_2 \cdot \vec{v}_2 \right) + \right. \\ \left. \frac{1}{r^5} \left( 5 \hat{n} \cdot \vec{S}_1 \hat{n} \cdot \vec{S}_2 (\hat{n} \cdot \vec{v}_2)^2 + 35 \hat{n} \cdot \vec{S}_1 \hat{n} \cdot \vec{S}_2 \hat{n} \cdot \vec{v}_1 \hat{n} \cdot \vec{v}_2 - 5 \hat{n} \cdot \vec{S}_2 \vec{S}_1 \cdot \vec{v}_1 \hat{n} \cdot \vec{v}_2 - \hat{n} \cdot \vec{S}_2 \vec{S}_1 \cdot \vec{v}_2 \hat{n} \cdot \vec{v}_2 - \right. \right. \\ \left. \left. 5 \hat{n} \cdot \vec{S}_1 \vec{S}_2 \cdot \vec{v}_1 \hat{n} \cdot \vec{v}_2 - 2 \hat{n} \cdot \vec{S}_1 \vec{S}_2 \cdot \vec{v}_2 \hat{n} \cdot \vec{v}_2 - 10 \hat{n} \cdot \vec{S}_2 \hat{n} \cdot \vec{v}_1 \vec{S}_1 \cdot \vec{v}_2 + 2 \vec{S}_1 \cdot \vec{v}_2 \vec{S}_2 \cdot \vec{v}_1 - \right. \right. \\ \left. \left. 2 \vec{S}_1 \cdot \vec{v}_2 \vec{S}_2 \cdot \vec{v}_1 \right) \right)$$

$$\begin{aligned}
& 5 \hat{n} \cdot \vec{S}_1 \hat{n} \cdot \vec{v}_1 \vec{S}_2 \cdot \vec{v}_2 + \vec{S}_1 \cdot \vec{v}_1 \vec{S}_2 \cdot \vec{v}_2 + \vec{S}_1 \cdot \vec{v}_2 \vec{S}_2 \cdot \vec{v}_2 - 5 \hat{n} \cdot \vec{S}_1 \hat{n} \cdot \vec{S}_2 \vec{v}_1 \cdot \vec{v}_2 - 3 \hat{n} \cdot \vec{S}_1 \hat{n} \cdot \vec{S}_2 \vec{v}_2 \cdot \vec{v}_2 \Big) + \\
& \pi^2 \left( \frac{\frac{15}{16} \vec{S}_1 \cdot \vec{S}_2 - \frac{45}{16} \hat{n} \cdot \vec{S}_1 \hat{n} \cdot \vec{S}_2}{r^3} + \frac{1}{r^4} \left( \frac{225}{16} \hat{n} \cdot \vec{S}_2 \hat{n} \cdot \vec{S}_1 \hat{n} \cdot \vec{v}_1 - \frac{45}{16} \vec{S}_1 \cdot \vec{S}_2 \hat{n} \cdot \vec{v}_1 - \frac{135}{16} \hat{n} \cdot \vec{S}_2 \hat{n} \cdot \vec{S}_1 \hat{n} \cdot \vec{v}_2 - \right. \right. \\
& \quad \frac{45}{8} \hat{n} \cdot \vec{S}_1 \hat{n} \cdot \vec{S}_2 \hat{n} \cdot \vec{v}_2 + \frac{9}{8} \hat{n} \cdot \vec{v}_2 \vec{S}_1 \cdot \vec{S}_2 + \frac{9}{8} \hat{n} \cdot \vec{S}_2 \vec{S}_1 \cdot \vec{v}_2 - \frac{45}{16} \hat{n} \cdot \vec{S}_1 \vec{S}_2 \cdot \vec{v}_1 + \frac{27}{16} \hat{n} \cdot \vec{S}_1 \vec{S}_2 \cdot \vec{v}_2 + \\
& \quad \left. \frac{27}{16} \hat{n} \cdot \vec{v}_2 \vec{S}_1 \cdot \vec{S}_2 - \frac{45}{16} \hat{n} \cdot \vec{S}_2 \vec{S}_1 \cdot \vec{v}_1 + \frac{27}{16} \hat{n} \cdot \vec{S}_2 \vec{S}_1 \cdot \vec{v}_2 + \frac{9}{8} \hat{n} \cdot \vec{S}_1 \vec{S}_2 \cdot \vec{v}_2 \right) + \frac{1}{r^5} \\
& \quad \left( -\frac{1575}{128} \hat{n} \cdot \vec{S}_1 \hat{n} \cdot \vec{S}_2 (\hat{n} \cdot \vec{v}_2)^2 + \frac{225}{128} \vec{S}_1 \cdot \vec{S}_2 (\hat{n} \cdot \vec{v}_2)^2 + \frac{315}{8} \hat{n} \cdot \vec{S}_1 \hat{n} \cdot \vec{S}_2 \hat{n} \cdot \vec{v}_1 \hat{n} \cdot \vec{v}_2 - \frac{45}{8} \hat{n} \cdot \vec{v}_1 \vec{S}_1 \cdot \vec{S}_2 \hat{n} \cdot \vec{v}_2 - \right. \\
& \quad \frac{45}{8} \hat{n} \cdot \vec{S}_2 \vec{S}_1 \cdot \vec{v}_1 \hat{n} \cdot \vec{v}_2 + \frac{225}{64} \hat{n} \cdot \vec{S}_2 \vec{S}_1 \cdot \vec{v}_2 \hat{n} \cdot \vec{v}_2 - \frac{45}{8} \hat{n} \cdot \vec{S}_1 \vec{S}_2 \cdot \vec{v}_1 \hat{n} \cdot \vec{v}_2 + \frac{225}{64} \hat{n} \cdot \vec{S}_1 \vec{S}_2 \cdot \vec{v}_2 \hat{n} \cdot \vec{v}_2 - \\
& \quad \frac{45}{8} \hat{n} \cdot \vec{S}_2 \hat{n} \cdot \vec{v}_1 \vec{S}_1 \cdot \vec{v}_2 + \frac{9}{8} \vec{S}_1 \cdot \vec{v}_2 \vec{S}_2 \cdot \vec{v}_1 - \frac{45}{8} \hat{n} \cdot \vec{S}_1 \hat{n} \cdot \vec{v}_1 \vec{S}_2 \cdot \vec{v}_2 + \frac{9}{8} \vec{S}_1 \cdot \vec{v}_1 \vec{S}_2 \cdot \vec{v}_2 - \frac{45}{64} \vec{S}_1 \cdot \vec{v}_2 \vec{S}_2 \cdot \vec{v}_2 - \\
& \quad \left. \frac{45}{8} \hat{n} \cdot \vec{S}_1 \hat{n} \cdot \vec{S}_2 \vec{v}_1 \cdot \vec{v}_2 + \frac{9}{8} \vec{S}_1 \cdot \vec{S}_2 \vec{v}_1 \cdot \vec{v}_2 + \frac{225}{128} \hat{n} \cdot \vec{S}_1 \hat{n} \cdot \vec{S}_2 \vec{v}_2 \cdot \vec{v}_2 - \frac{45}{128} \vec{S}_1 \cdot \vec{S}_2 \vec{v}_2 \cdot \vec{v}_2 \right) \Bigg\} m_1 m_2 \Bigg\}
\end{aligned}$$

{DiagS1S2[3, 9, 43],

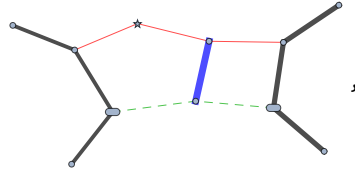

$$\begin{aligned}
& G^3 \left( \frac{1}{r^4} \left( \frac{71}{2} \hat{n} \cdot \vec{S}_2 \hat{n} \cdot \vec{S}_1 \hat{n} \cdot \vec{v}_2 + \frac{71}{2} \hat{n} \cdot \vec{S}_1 \hat{n} \cdot \vec{S}_2 \hat{n} \cdot \vec{v}_2 - \frac{11}{2} \vec{S}_1 \cdot \vec{S}_2 \hat{n} \cdot \vec{v}_2 - \right. \right. \\
& \quad \frac{11}{2} \vec{S}_1 \cdot \vec{S}_2 \hat{n} \cdot \vec{v}_2 - \frac{17}{2} \hat{n} \cdot \vec{S}_2 \vec{S}_1 \cdot \vec{v}_2 - \frac{17}{2} \hat{n} \cdot \vec{S}_1 \vec{S}_2 \cdot \vec{v}_2 - \frac{17}{2} \hat{n} \cdot \vec{S}_2 \vec{S}_1 \cdot \vec{v}_2 - \frac{17}{2} \hat{n} \cdot \vec{S}_1 \vec{S}_2 \cdot \vec{v}_2 \Big) + \frac{1}{r^5} \\
& \quad \left( \frac{5107}{24} \hat{n} \cdot \vec{S}_1 \hat{n} \cdot \vec{S}_2 (\hat{n} \cdot \vec{v}_2)^2 - \frac{397}{24} \vec{S}_1 \cdot \vec{S}_2 (\hat{n} \cdot \vec{v}_2)^2 - \frac{497}{2} \hat{n} \cdot \vec{S}_1 \hat{n} \cdot \vec{S}_2 \hat{n} \cdot \vec{v}_1 \hat{n} \cdot \vec{v}_2 + \frac{55}{2} \hat{n} \cdot \vec{v}_1 \vec{S}_1 \cdot \vec{S}_2 \hat{n} \cdot \vec{v}_2 + \right. \\
& \quad \frac{71}{2} \hat{n} \cdot \vec{S}_2 \vec{S}_1 \cdot \vec{v}_1 \hat{n} \cdot \vec{v}_2 - \frac{853}{12} \hat{n} \cdot \vec{S}_2 \vec{S}_1 \cdot \vec{v}_2 \hat{n} \cdot \vec{v}_2 + \frac{71}{2} \hat{n} \cdot \vec{S}_1 \vec{S}_2 \cdot \vec{v}_1 \hat{n} \cdot \vec{v}_2 - \frac{793}{12} \hat{n} \cdot \vec{S}_1 \vec{S}_2 \cdot \vec{v}_2 \hat{n} \cdot \vec{v}_2 + \\
& \quad 9 \hat{n} \times \vec{S}_1 \cdot \vec{v}_2 \hat{n} \times \vec{S}_2 \cdot \vec{v}_2 + \frac{85}{2} \hat{n} \cdot \vec{S}_2 \hat{n} \cdot \vec{v}_1 \vec{S}_1 \cdot \vec{v}_2 - \frac{17}{2} \vec{S}_1 \cdot \vec{v}_2 \vec{S}_2 \cdot \vec{v}_1 + \frac{85}{2} \hat{n} \cdot \vec{S}_1 \hat{n} \cdot \vec{v}_1 \vec{S}_2 \cdot \vec{v}_2 - \frac{17}{2} \vec{S}_1 \cdot \vec{v}_1 \vec{S}_2 \cdot \vec{v}_2 + \\
& \quad \left. \frac{257}{12} \vec{S}_1 \cdot \vec{v}_2 \vec{S}_2 \cdot \vec{v}_2 + \frac{71}{2} \hat{n} \cdot \vec{S}_1 \hat{n} \cdot \vec{S}_2 \vec{v}_1 \cdot \vec{v}_2 - \frac{11}{2} \vec{S}_1 \cdot \vec{S}_2 \vec{v}_1 \cdot \vec{v}_2 - \frac{1045}{24} \hat{n} \cdot \vec{S}_1 \hat{n} \cdot \vec{S}_2 \vec{v}_2 \cdot \vec{v}_2 + \frac{17}{24} \vec{S}_1 \cdot \vec{S}_2 \vec{v}_2 \cdot \vec{v}_2 \right) + \\
& \quad \pi^2 \left( \frac{1}{r^4} \left( -\frac{45}{16} \hat{n} \cdot \vec{S}_2 \hat{n} \cdot \vec{S}_1 \hat{n} \cdot \vec{v}_2 - \frac{45}{16} \hat{n} \cdot \vec{S}_1 \hat{n} \cdot \vec{S}_2 \hat{n} \cdot \vec{v}_2 + \frac{9}{16} \vec{S}_1 \cdot \vec{S}_2 \hat{n} \cdot \vec{v}_2 + \frac{9}{16} \vec{S}_1 \cdot \vec{S}_2 \hat{n} \cdot \vec{v}_2 + \right. \right. \\
& \quad \frac{9}{16} \hat{n} \cdot \vec{S}_2 \vec{S}_1 \cdot \vec{v}_2 + \frac{9}{16} \hat{n} \cdot \vec{S}_1 \vec{S}_2 \cdot \vec{v}_2 + \frac{9}{16} \hat{n} \cdot \vec{S}_2 \vec{S}_1 \cdot \vec{v}_2 + \frac{9}{16} \hat{n} \cdot \vec{S}_1 \vec{S}_2 \cdot \vec{v}_2 \Big) + \frac{1}{r^5} \\
& \quad \left( -\frac{1995}{128} \hat{n} \cdot \vec{S}_1 \hat{n} \cdot \vec{S}_2 (\hat{n} \cdot \vec{v}_2)^2 + \frac{285}{128} \vec{S}_1 \cdot \vec{S}_2 (\hat{n} \cdot \vec{v}_2)^2 + \frac{315}{16} \hat{n} \cdot \vec{S}_1 \hat{n} \cdot \vec{S}_2 \hat{n} \cdot \vec{v}_1 \hat{n} \cdot \vec{v}_2 - \frac{45}{16} \hat{n} \cdot \vec{v}_1 \vec{S}_1 \cdot \vec{S}_2 \hat{n} \cdot \vec{v}_2 - \right. \\
& \quad \frac{45}{16} \hat{n} \cdot \vec{S}_2 \vec{S}_1 \cdot \vec{v}_1 \hat{n} \cdot \vec{v}_2 + \frac{285}{64} \hat{n} \cdot \vec{S}_2 \vec{S}_1 \cdot \vec{v}_2 \hat{n} \cdot \vec{v}_2 - \frac{45}{16} \hat{n} \cdot \vec{S}_1 \vec{S}_2 \cdot \vec{v}_1 \hat{n} \cdot \vec{v}_2 + \frac{285}{64} \hat{n} \cdot \vec{S}_1 \vec{S}_2 \cdot \vec{v}_2 \hat{n} \cdot \vec{v}_2 - \\
& \quad \frac{45}{16} \hat{n} \cdot \vec{S}_2 \hat{n} \cdot \vec{v}_1 \vec{S}_1 \cdot \vec{v}_2 + \frac{9}{16} \vec{S}_1 \cdot \vec{v}_2 \vec{S}_2 \cdot \vec{v}_1 - \frac{45}{16} \hat{n} \cdot \vec{S}_1 \hat{n} \cdot \vec{v}_1 \vec{S}_2 \cdot \vec{v}_2 + \frac{9}{16} \vec{S}_1 \cdot \vec{v}_1 \vec{S}_2 \cdot \vec{v}_2 - \frac{57}{64} \vec{S}_1 \cdot \vec{v}_2 \vec{S}_2 \cdot \vec{v}_2 - \\
& \quad \left. \frac{45}{16} \hat{n} \cdot \vec{S}_1 \hat{n} \cdot \vec{S}_2 \vec{v}_1 \cdot \vec{v}_2 + \frac{9}{16} \vec{S}_1 \cdot \vec{S}_2 \vec{v}_1 \cdot \vec{v}_2 + \frac{285}{128} \hat{n} \cdot \vec{S}_1 \hat{n} \cdot \vec{S}_2 \vec{v}_2 \cdot \vec{v}_2 - \frac{57}{128} \vec{S}_1 \cdot \vec{S}_2 \vec{v}_2 \cdot \vec{v}_2 \right) \Bigg\} m_1 m_2 \Bigg\}
\end{aligned}$$



{DiagS1S2[3, 9, 44],

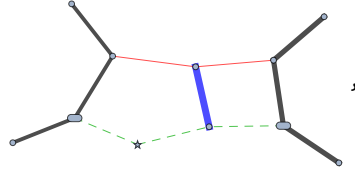

,

$$\begin{aligned}
 & G^3 \left( \frac{\frac{8}{3} \vec{S}_1 \cdot \vec{S}_2 - 12 \hat{n} \cdot \vec{S}_1 \hat{n} \cdot \vec{S}_2}{r^3} + \frac{1}{r^4} \left( 60 \hat{n} \cdot \vec{S}_2 \hat{n} \cdot \vec{S}_1 \hat{n} \cdot \vec{v}_1 - 8 \vec{S}_1 \cdot \vec{S}_2 \hat{n} \cdot \vec{v}_1 - \right. \right. \\
 & 33 \hat{n} \cdot \vec{S}_2 \hat{n} \cdot \vec{S}_1 \hat{n} \cdot \vec{v}_2 - 27 \hat{n} \cdot \vec{S}_1 \hat{n} \cdot \vec{S}_2 \hat{n} \cdot \vec{v}_2 + 3 \hat{n} \cdot \vec{v}_2 \vec{S}_1 \cdot \vec{S}_2 + 6 \hat{n} \cdot \vec{S}_2 \vec{S}_1 \cdot \vec{v}_2 - 12 \hat{n} \cdot \vec{S}_1 \vec{S}_2 \cdot \vec{v}_1 + \\
 & 6 \hat{n} \cdot \vec{S}_1 \vec{S}_2 \cdot \vec{v}_2 + 5 \hat{n} \cdot \vec{v}_2 \vec{S}_1 \cdot \vec{S}_2 - 12 \hat{n} \cdot \vec{S}_2 \vec{S}_1 \cdot \vec{v}_1 + 6 \hat{n} \cdot \vec{S}_2 \vec{S}_1 \cdot \vec{v}_2 + 6 \hat{n} \cdot \vec{S}_1 \vec{S}_2 \cdot \vec{v}_2 \left. \right) + \frac{1}{r^5} \\
 & \left( -\frac{163}{2} \hat{n} \cdot \vec{S}_1 \hat{n} \cdot \vec{S}_2 (\hat{n} \cdot \vec{v}_2)^2 + \frac{35}{2} \vec{S}_1 \cdot \vec{S}_2 (\hat{n} \cdot \vec{v}_2)^2 + 189 \hat{n} \cdot \vec{S}_1 \hat{n} \cdot \vec{S}_2 \hat{n} \cdot \vec{v}_1 \hat{n} \cdot \vec{v}_2 - 15 \hat{n} \cdot \vec{v}_1 \vec{S}_1 \cdot \vec{S}_2 \hat{n} \cdot \vec{v}_2 - \right. \\
 & 27 \hat{n} \cdot \vec{S}_2 \vec{S}_1 \cdot \vec{v}_1 \hat{n} \cdot \vec{v}_2 + 17 \hat{n} \cdot \vec{S}_2 \vec{S}_1 \cdot \vec{v}_2 \hat{n} \cdot \vec{v}_2 - 27 \hat{n} \cdot \vec{S}_1 \vec{S}_2 \cdot \vec{v}_1 \hat{n} \cdot \vec{v}_2 + 22 \hat{n} \cdot \vec{S}_1 \vec{S}_2 \cdot \vec{v}_2 \hat{n} \cdot \vec{v}_2 + \\
 & 9 \hat{n} \times \vec{S}_1 \cdot \vec{v}_2 \hat{n} \times \vec{S}_2 \cdot \vec{v}_2 - 30 \hat{n} \cdot \vec{S}_2 \hat{n} \cdot \vec{v}_1 \vec{S}_1 \cdot \vec{v}_2 + 6 \vec{S}_1 \cdot \vec{v}_2 \vec{S}_2 \cdot \vec{v}_1 - 30 \hat{n} \cdot \vec{S}_1 \hat{n} \cdot \vec{v}_1 \vec{S}_2 \cdot \vec{v}_2 + 6 \vec{S}_1 \cdot \vec{v}_1 \vec{S}_2 \cdot \vec{v}_2 + \\
 & 3 \vec{S}_1 \cdot \vec{v}_2 \vec{S}_2 \cdot \vec{v}_2 - 27 \hat{n} \cdot \vec{S}_1 \hat{n} \cdot \vec{S}_2 \vec{v}_1 \cdot \vec{v}_2 + 3 \vec{S}_1 \cdot \vec{S}_2 \vec{v}_1 \cdot \vec{v}_2 + \frac{5}{2} \hat{n} \cdot \vec{S}_1 \hat{n} \cdot \vec{S}_2 \vec{v}_2 \cdot \vec{v}_2 - \frac{17}{2} \vec{S}_1 \cdot \vec{S}_2 \vec{v}_2 \cdot \vec{v}_2 \left. \right) + \\
 & \pi^2 \left( \frac{\frac{3}{8} \hat{n} \cdot \vec{S}_1 \hat{n} \cdot \vec{S}_2 - \frac{1}{8} \vec{S}_1 \cdot \vec{S}_2}{r^3} + \frac{1}{r^4} \left( -\frac{15}{8} \hat{n} \cdot \vec{S}_2 \hat{n} \cdot \vec{S}_1 \hat{n} \cdot \vec{v}_1 + \frac{3}{8} \vec{S}_1 \cdot \vec{S}_2 \hat{n} \cdot \vec{v}_1 + \frac{15}{16} \hat{n} \cdot \vec{S}_2 \hat{n} \cdot \vec{S}_1 \hat{n} \cdot \vec{v}_2 + \right. \right. \\
 & \frac{15}{16} \hat{n} \cdot \vec{S}_1 \hat{n} \cdot \vec{S}_2 \hat{n} \cdot \vec{v}_2 - \frac{3}{16} \hat{n} \cdot \vec{v}_2 \vec{S}_1 \cdot \vec{S}_2 - \frac{3}{16} \hat{n} \cdot \vec{S}_2 \vec{S}_1 \cdot \vec{v}_2 + \frac{3}{8} \hat{n} \cdot \vec{S}_1 \vec{S}_2 \cdot \vec{v}_1 - \\
 & \frac{3}{16} \hat{n} \cdot \vec{S}_1 \vec{S}_2 \cdot \vec{v}_2 - \frac{3}{16} \hat{n} \cdot \vec{v}_2 \vec{S}_1 \cdot \vec{S}_2 + \frac{3}{8} \hat{n} \cdot \vec{S}_2 \vec{S}_1 \cdot \vec{v}_1 - \frac{3}{16} \hat{n} \cdot \vec{S}_2 \vec{S}_1 \cdot \vec{v}_2 - \frac{3}{16} \hat{n} \cdot \vec{S}_1 \vec{S}_2 \cdot \vec{v}_2 \left. \right) + \frac{1}{r^5} \\
 & \left( \frac{315}{64} \hat{n} \cdot \vec{S}_1 \hat{n} \cdot \vec{S}_2 (\hat{n} \cdot \vec{v}_2)^2 - \frac{45}{64} \vec{S}_1 \cdot \vec{S}_2 (\hat{n} \cdot \vec{v}_2)^2 - \frac{105}{16} \hat{n} \cdot \vec{S}_1 \hat{n} \cdot \vec{S}_2 \hat{n} \cdot \vec{v}_1 \hat{n} \cdot \vec{v}_2 + \frac{15}{16} \hat{n} \cdot \vec{v}_1 \vec{S}_1 \cdot \vec{S}_2 \hat{n} \cdot \vec{v}_2 + \right. \\
 & \frac{15}{16} \hat{n} \cdot \vec{S}_2 \vec{S}_1 \cdot \vec{v}_1 \hat{n} \cdot \vec{v}_2 - \frac{45}{32} \hat{n} \cdot \vec{S}_2 \vec{S}_1 \cdot \vec{v}_2 \hat{n} \cdot \vec{v}_2 + \frac{15}{16} \hat{n} \cdot \vec{S}_1 \vec{S}_2 \cdot \vec{v}_1 \hat{n} \cdot \vec{v}_2 - \frac{45}{32} \hat{n} \cdot \vec{S}_1 \vec{S}_2 \cdot \vec{v}_2 \hat{n} \cdot \vec{v}_2 + \\
 & \frac{15}{16} \hat{n} \cdot \vec{S}_2 \hat{n} \cdot \vec{v}_1 \vec{S}_1 \cdot \vec{v}_2 - \frac{3}{16} \vec{S}_1 \cdot \vec{v}_2 \vec{S}_2 \cdot \vec{v}_1 + \frac{15}{16} \hat{n} \cdot \vec{S}_1 \hat{n} \cdot \vec{v}_1 \vec{S}_2 \cdot \vec{v}_2 - \frac{3}{16} \vec{S}_1 \cdot \vec{v}_1 \vec{S}_2 \cdot \vec{v}_2 + \frac{9}{32} \vec{S}_1 \cdot \vec{v}_2 \vec{S}_2 \cdot \vec{v}_2 + \\
 & \left. \left. \frac{15}{16} \hat{n} \cdot \vec{S}_1 \hat{n} \cdot \vec{S}_2 \vec{v}_1 \cdot \vec{v}_2 - \frac{3}{16} \vec{S}_1 \cdot \vec{S}_2 \vec{v}_1 \cdot \vec{v}_2 - \frac{45}{64} \hat{n} \cdot \vec{S}_1 \hat{n} \cdot \vec{S}_2 \vec{v}_2 \cdot \vec{v}_2 + \frac{9}{64} \vec{S}_1 \cdot \vec{S}_2 \vec{v}_2 \cdot \vec{v}_2 \right) \right) \Bigg\} m_1 m_2 \}
 \end{aligned}$$
